# Supplementary material for: Pebbles, graphs and equilibria: higher order shape descriptors for sedimentary particles
Source: arXiv:2303.05285 ancillary file (2023-03-09)
Supplement: Supplementary file 1 [file catalog.pdf]

| Line | Pebble                                                                              | Point of origin                                         |                                                                             |                                                      | Material                       | Reeb-graph                                                                            | Quasi-dual<br>of the<br>Morse–Smale<br>graph                                          | Master<br>graph                                                                       |
|------|-------------------------------------------------------------------------------------|---------------------------------------------------------|-----------------------------------------------------------------------------|------------------------------------------------------|--------------------------------|---------------------------------------------------------------------------------------|---------------------------------------------------------------------------------------|---------------------------------------------------------------------------------------|
|      |                                                                                     | Weight                                                  | Volume                                                                      | Surface area                                         |                                |                                                                                       |                                                                                       |                                                                                       |
|      |                                                                                     | a                                                       | b                                                                           | c                                                    |                                |                                                                                       |                                                                                       |                                                                                       |
|      |                                                                                     | y <sup>1</sup><br>Measured<br>S                         | y <sup>2</sup><br>U                                                         | Zingg class<br>Computed<br>S                         |                                |                                                                                       |                                                                                       |                                                                                       |
| 1.   | 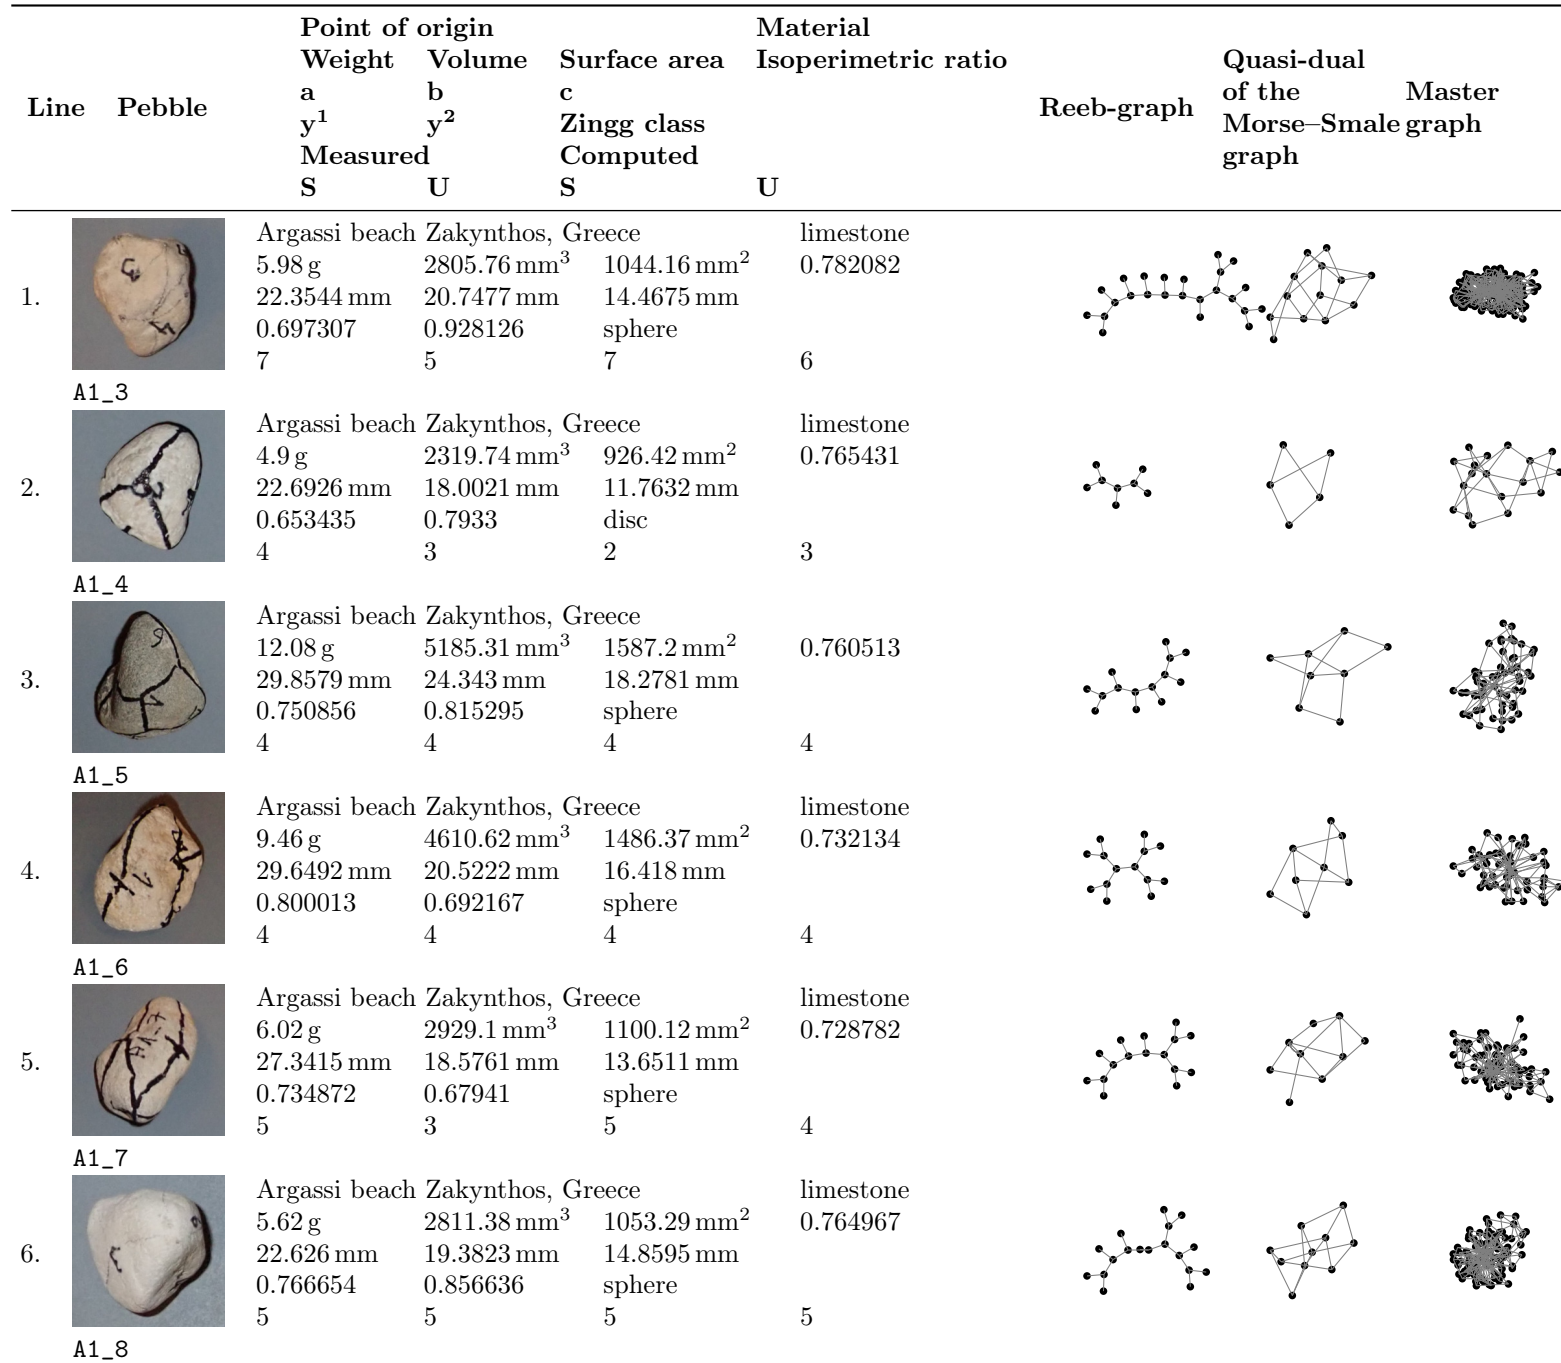   | Argassi beach<br>5.98 g<br>22.3544 mm<br>0.697307<br>7  | Zakynthos, Greece<br>2805.76 mm <sup>3</sup><br>20.7477 mm<br>0.928126<br>5 | 1044.16 mm <sup>2</sup><br>14.4675 mm<br>sphere<br>7 | limestone<br>0.782082<br><br>6 | 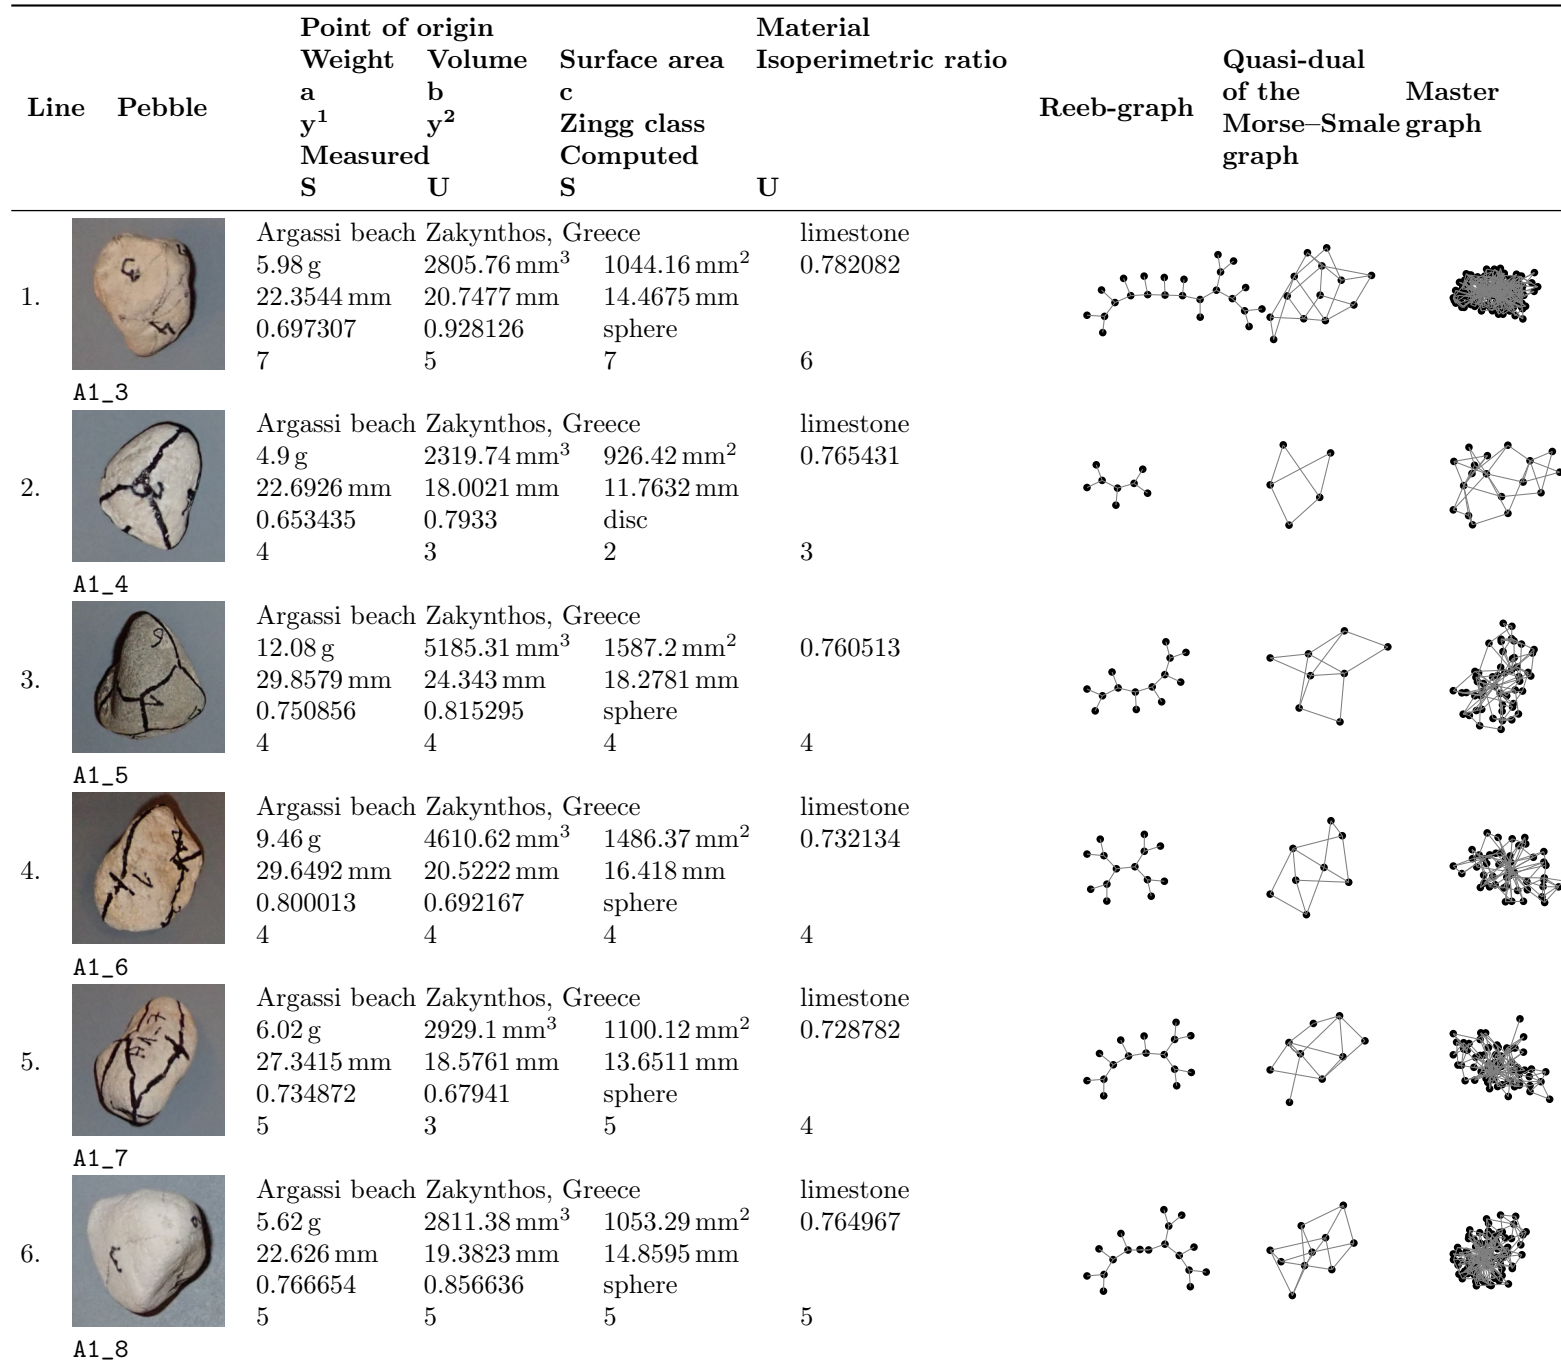   | 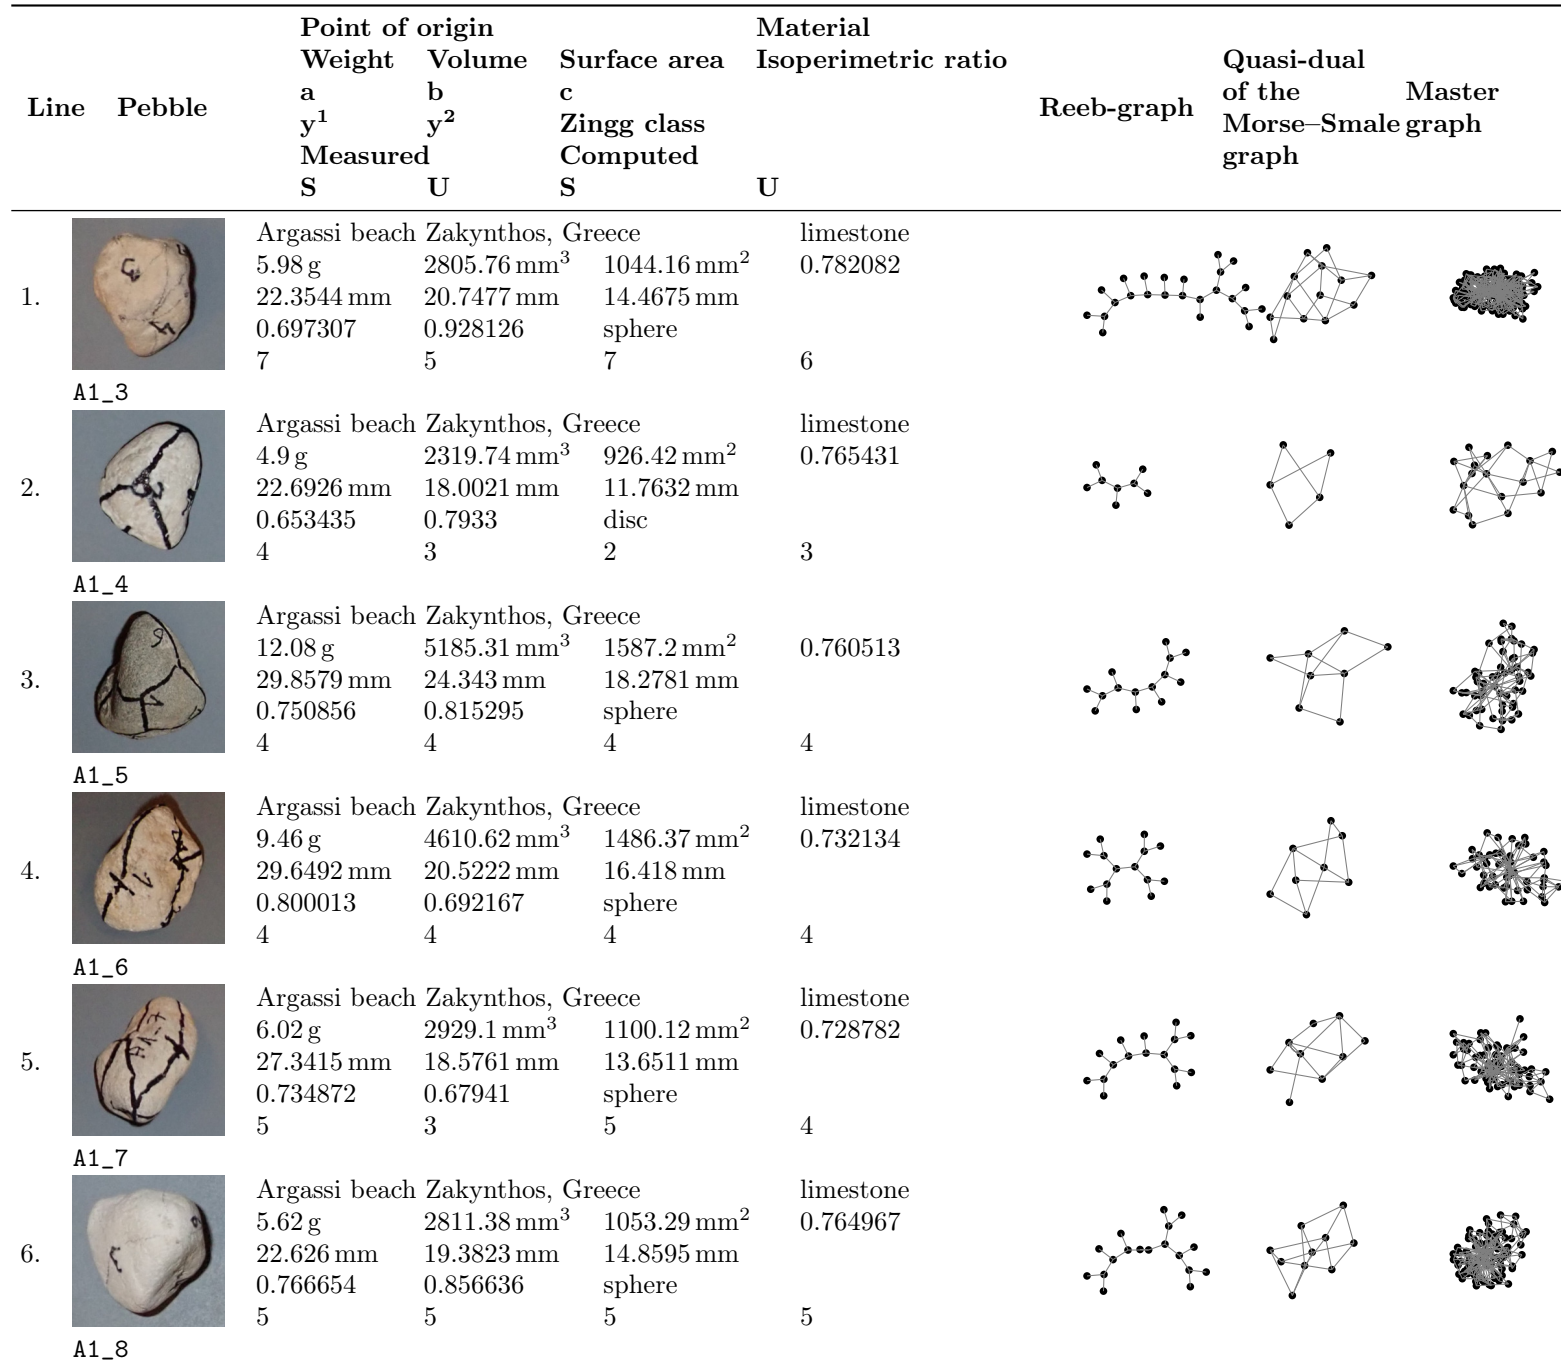   |                                                                                       |
| A1_3 |                                                                                     |                                                         |                                                                             |                                                      |                                |                                                                                       |                                                                                       |                                                                                       |
| 2.   | 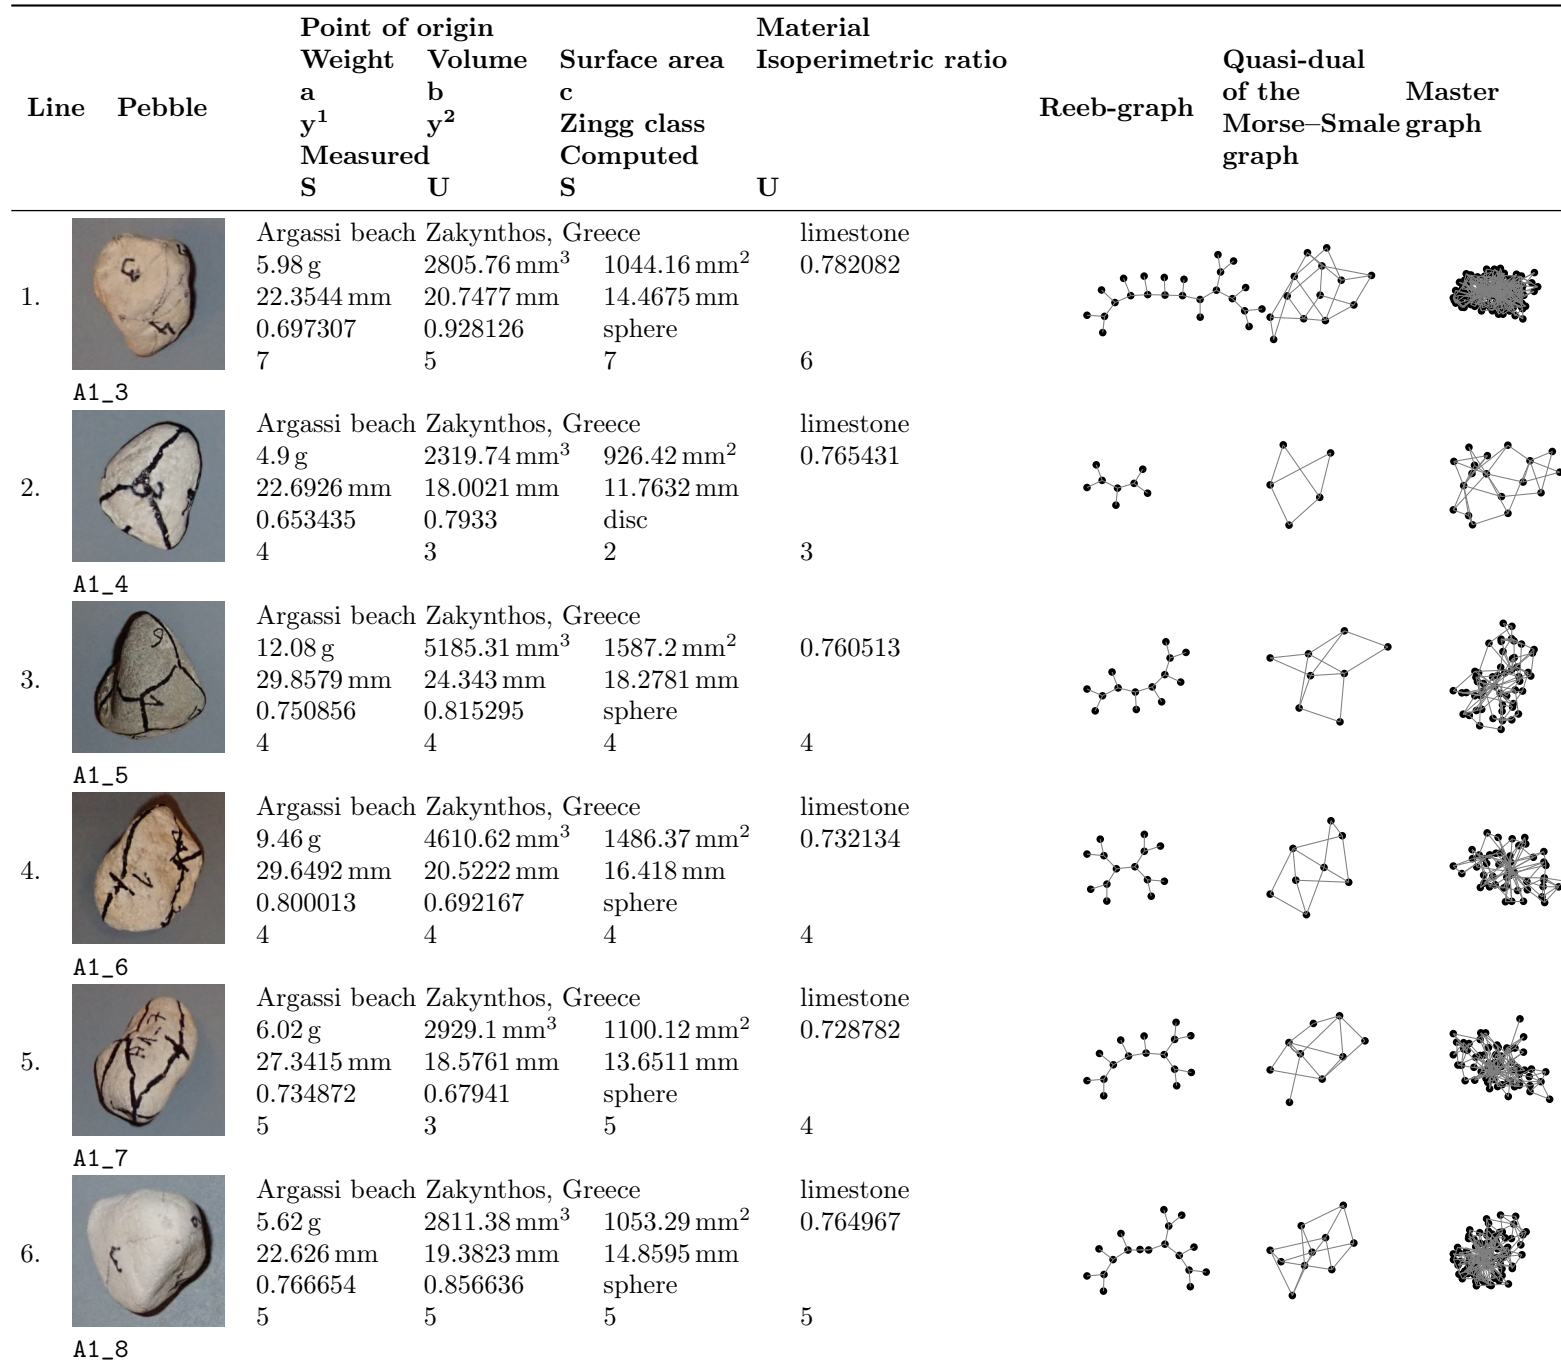   | Argassi beach<br>4.9 g<br>22.6926 mm<br>0.653435<br>4   | Zakynthos, Greece<br>2319.74 mm <sup>3</sup><br>18.0021 mm<br>0.7933<br>3   | 926.42 mm <sup>2</sup><br>11.7632 mm<br>disc<br>2    | limestone<br>0.765431<br><br>3 | 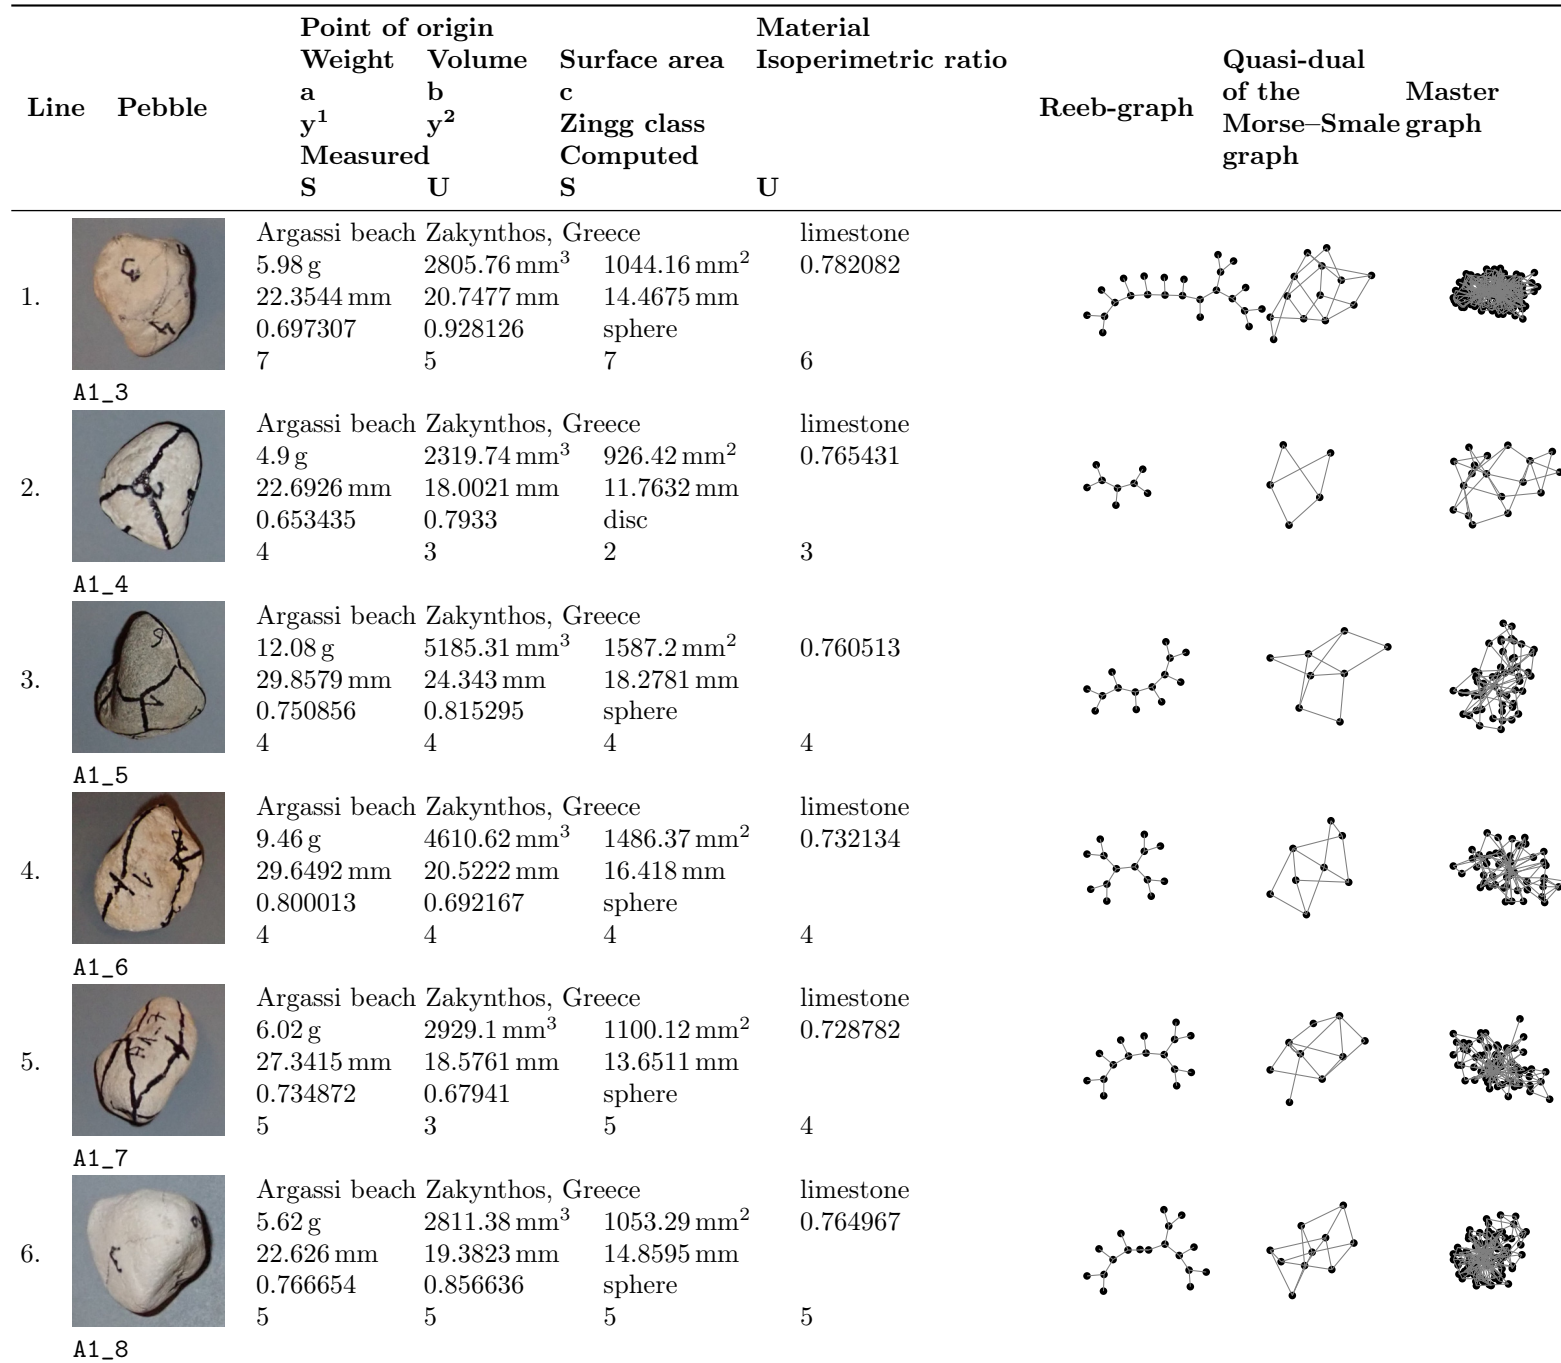   | 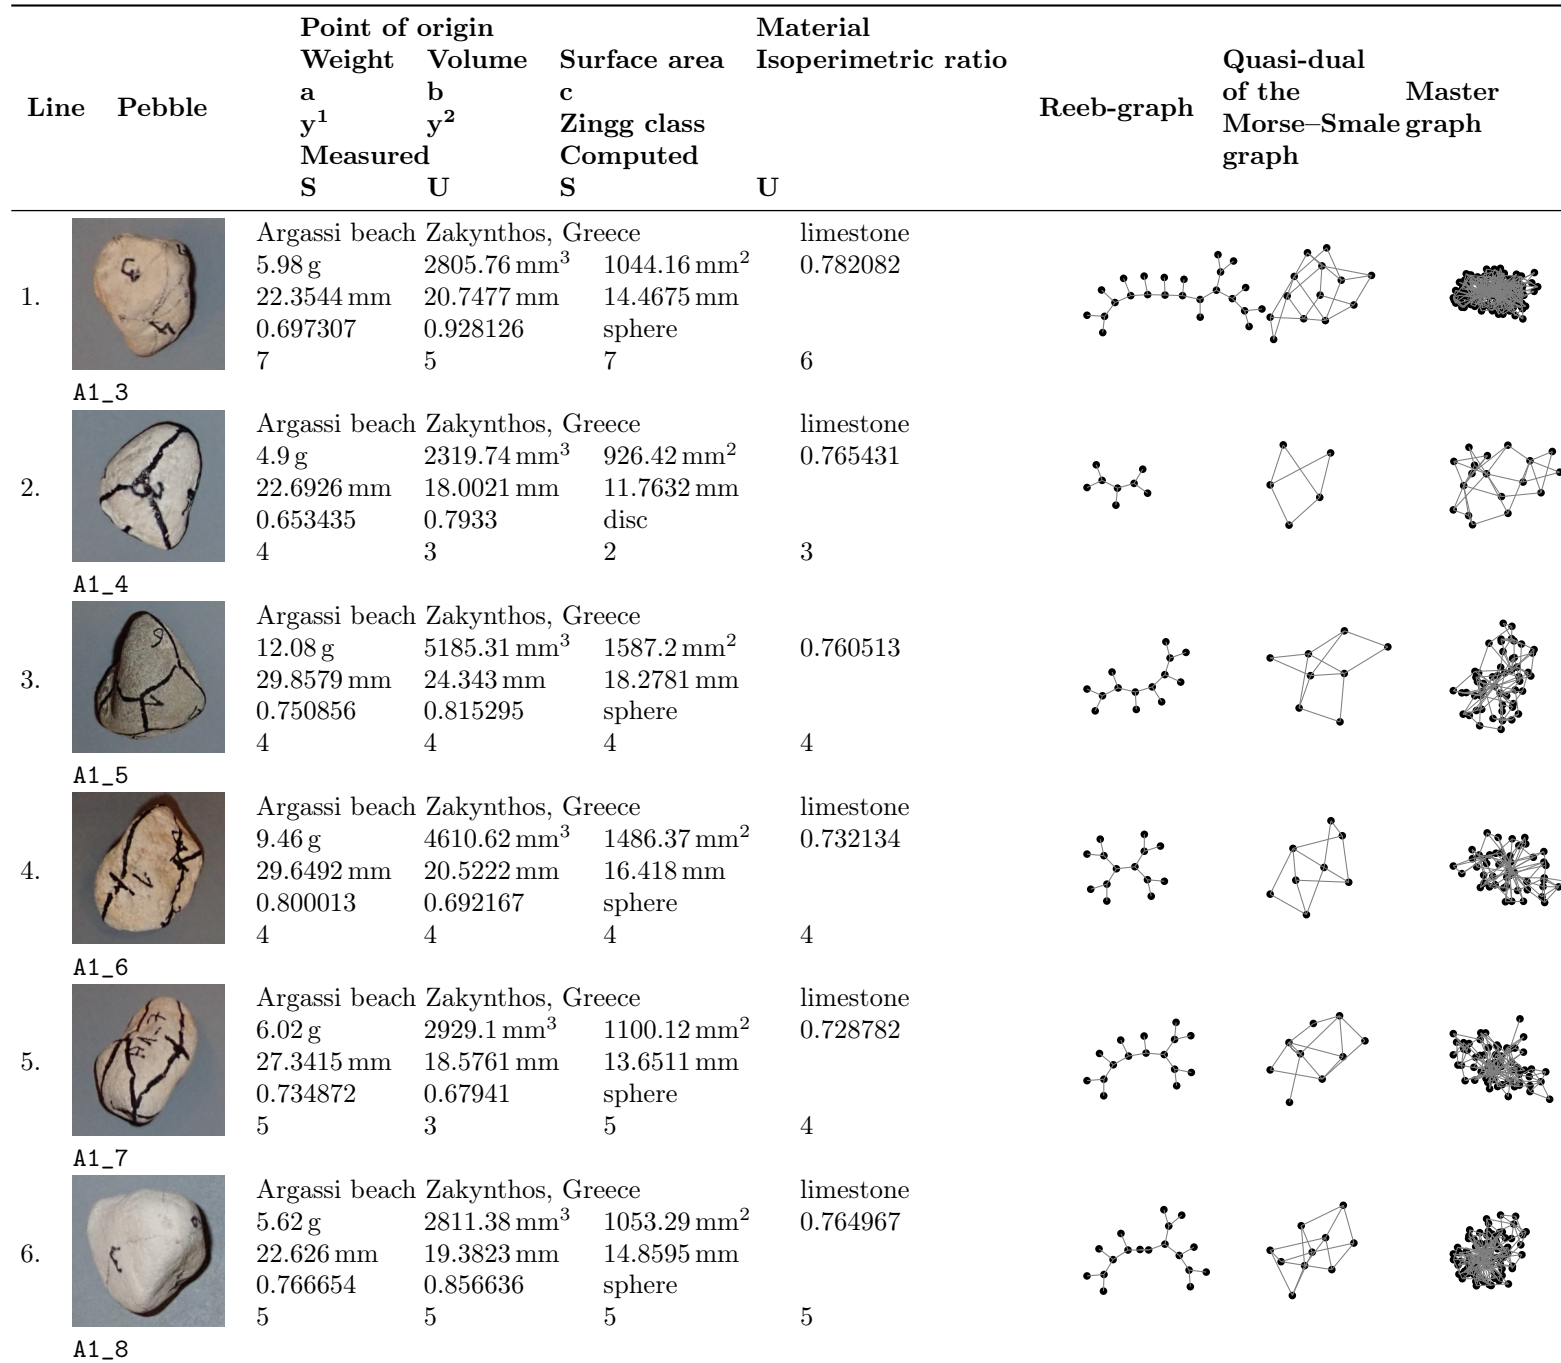   | 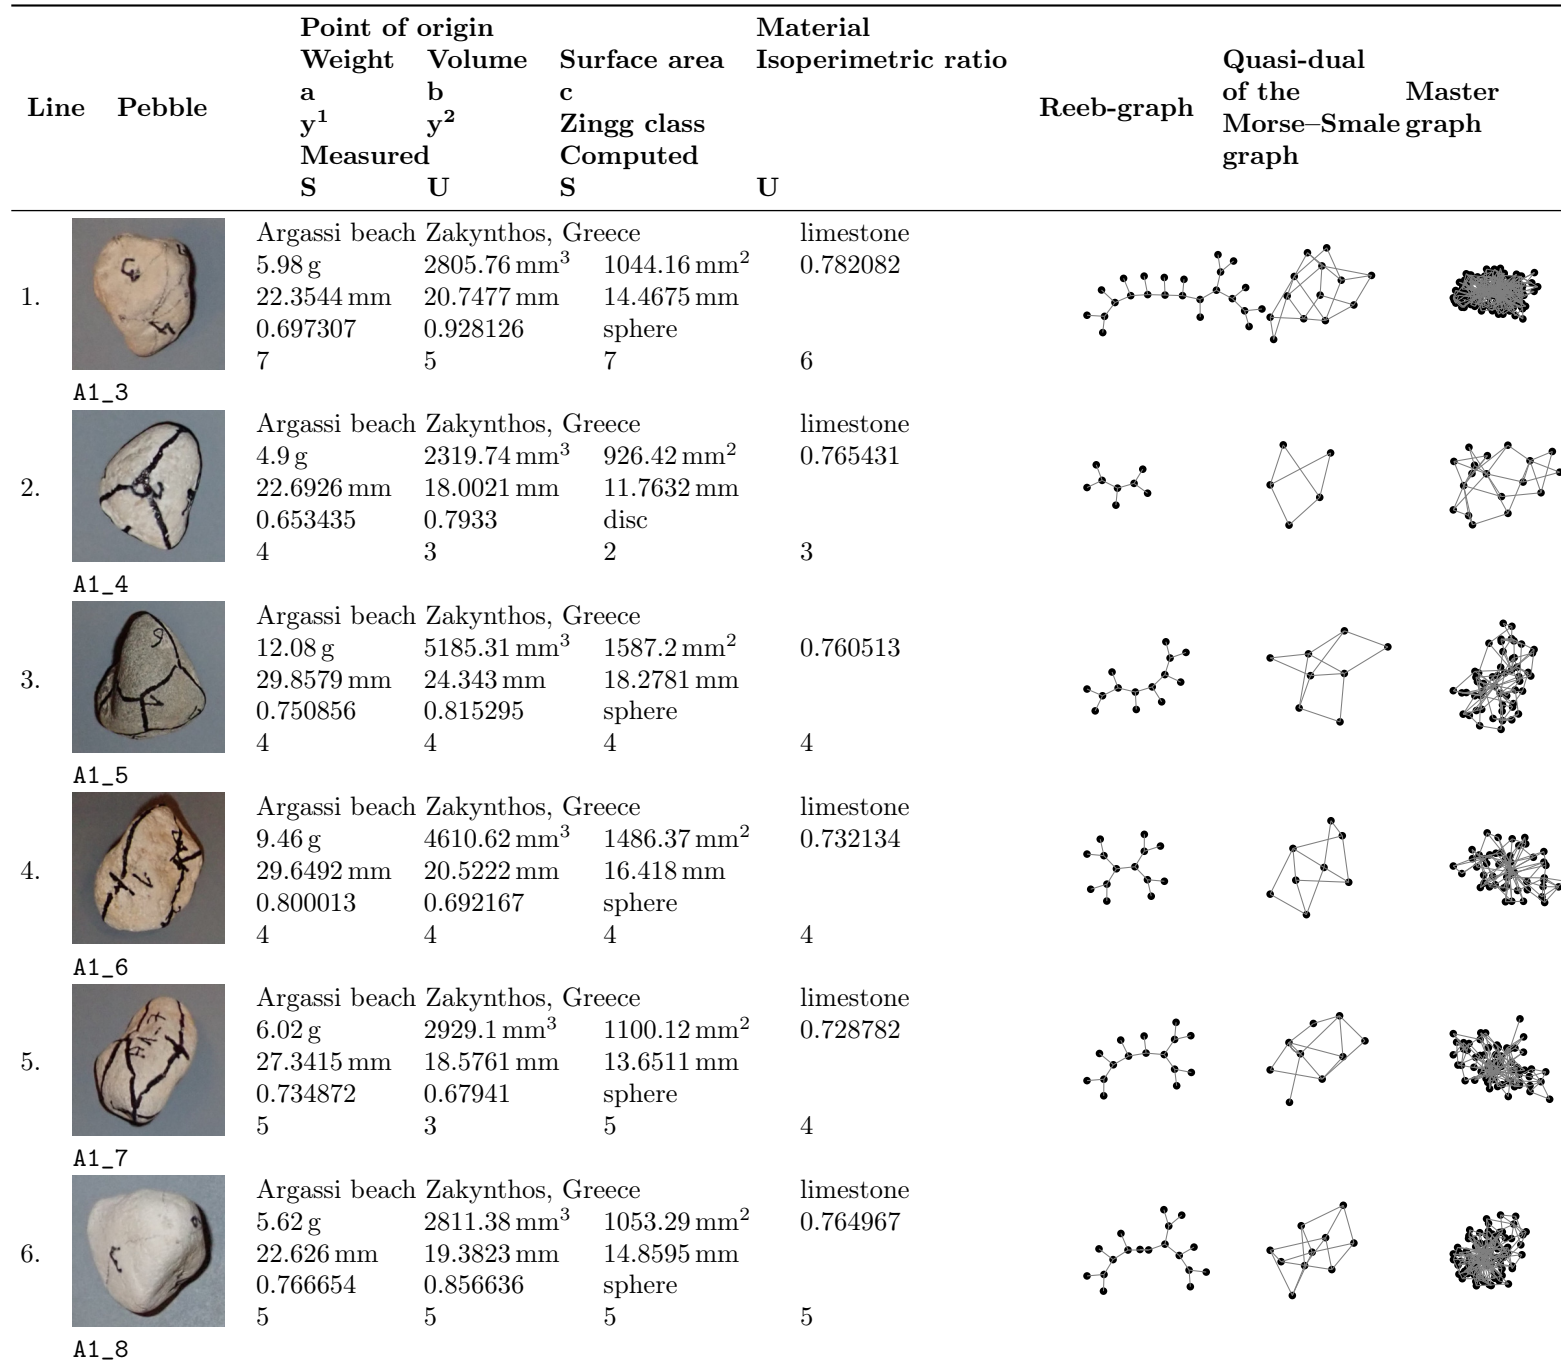   |
| A1_4 |                                                                                     |                                                         |                                                                             |                                                      |                                |                                                                                       |                                                                                       |                                                                                       |
| 3.   | 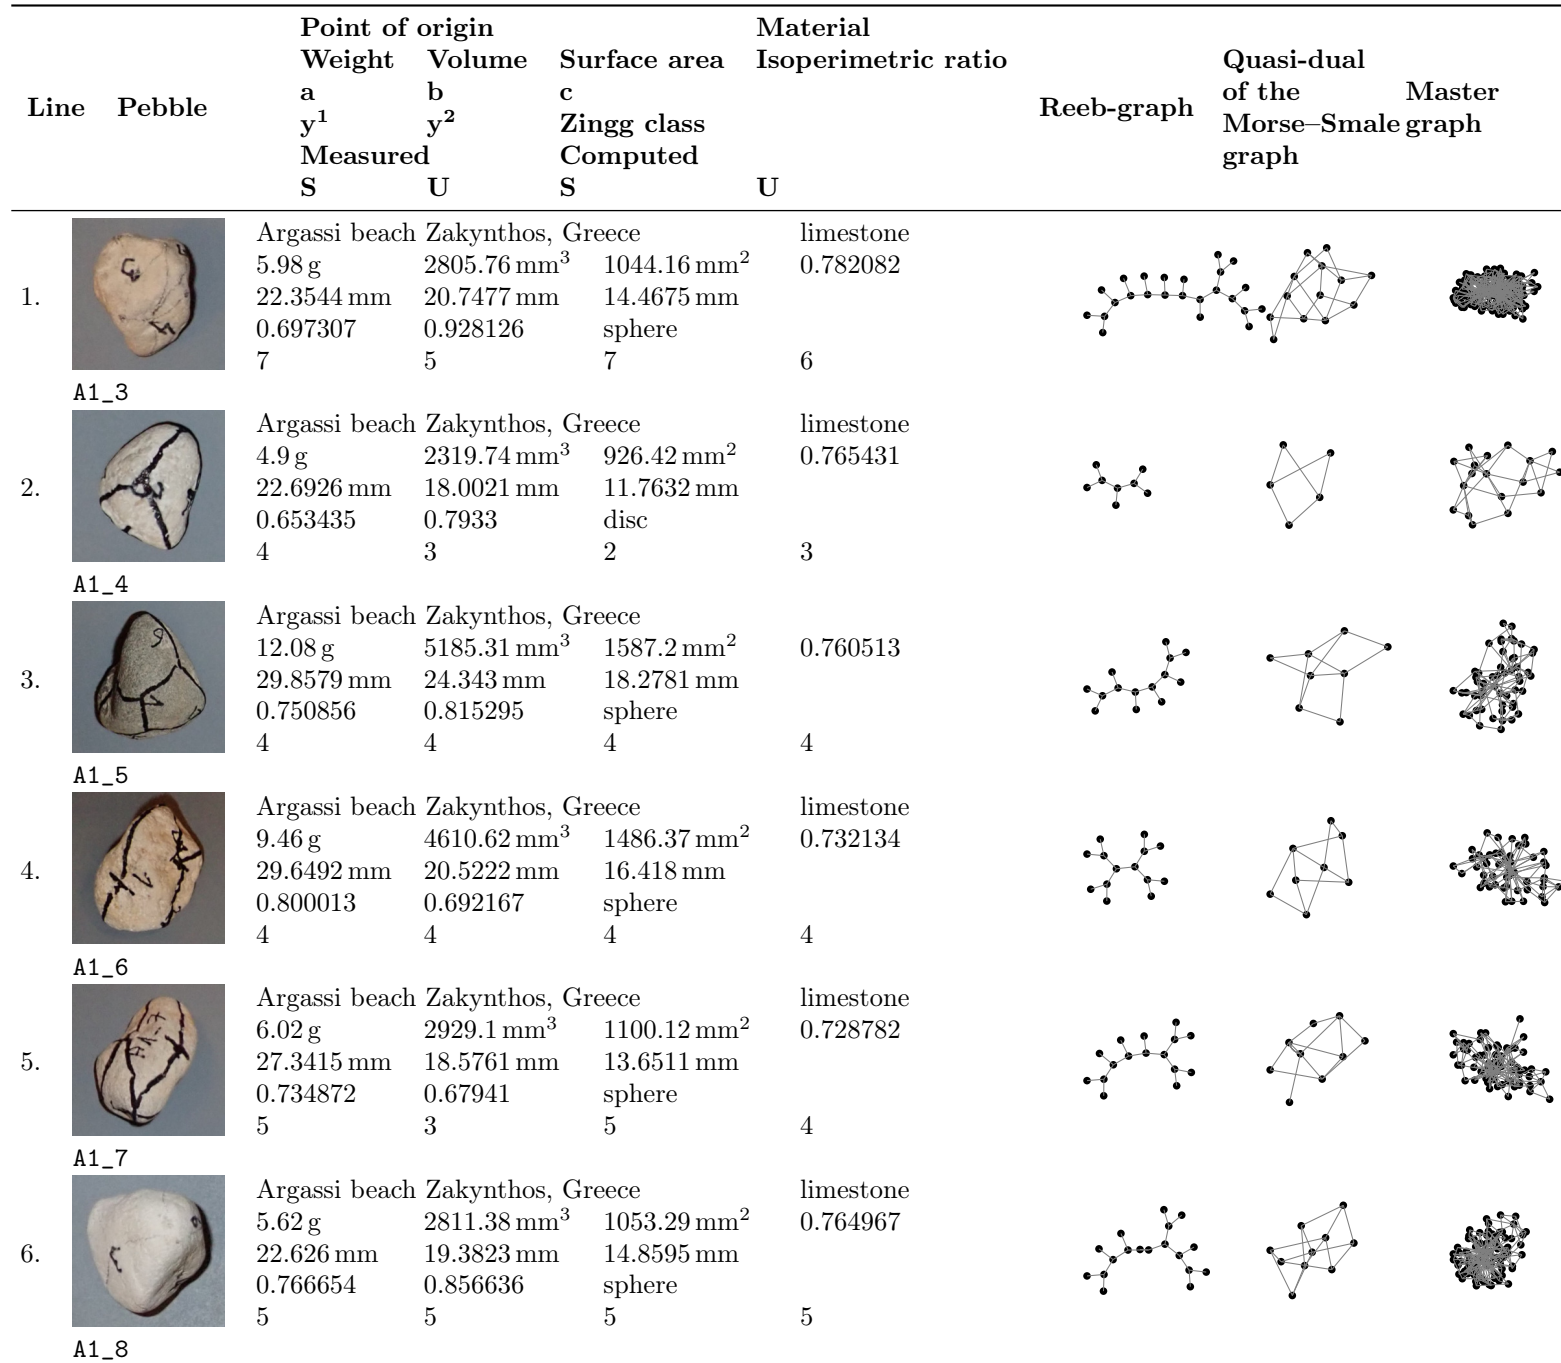   | Argassi beach<br>12.08 g<br>29.8579 mm<br>0.750856<br>4 | Zakynthos, Greece<br>5185.31 mm <sup>3</sup><br>24.343 mm<br>0.815295<br>4  | 1587.2 mm <sup>2</sup><br>18.2781 mm<br>sphere<br>4  | 0.760513<br><br>4              | 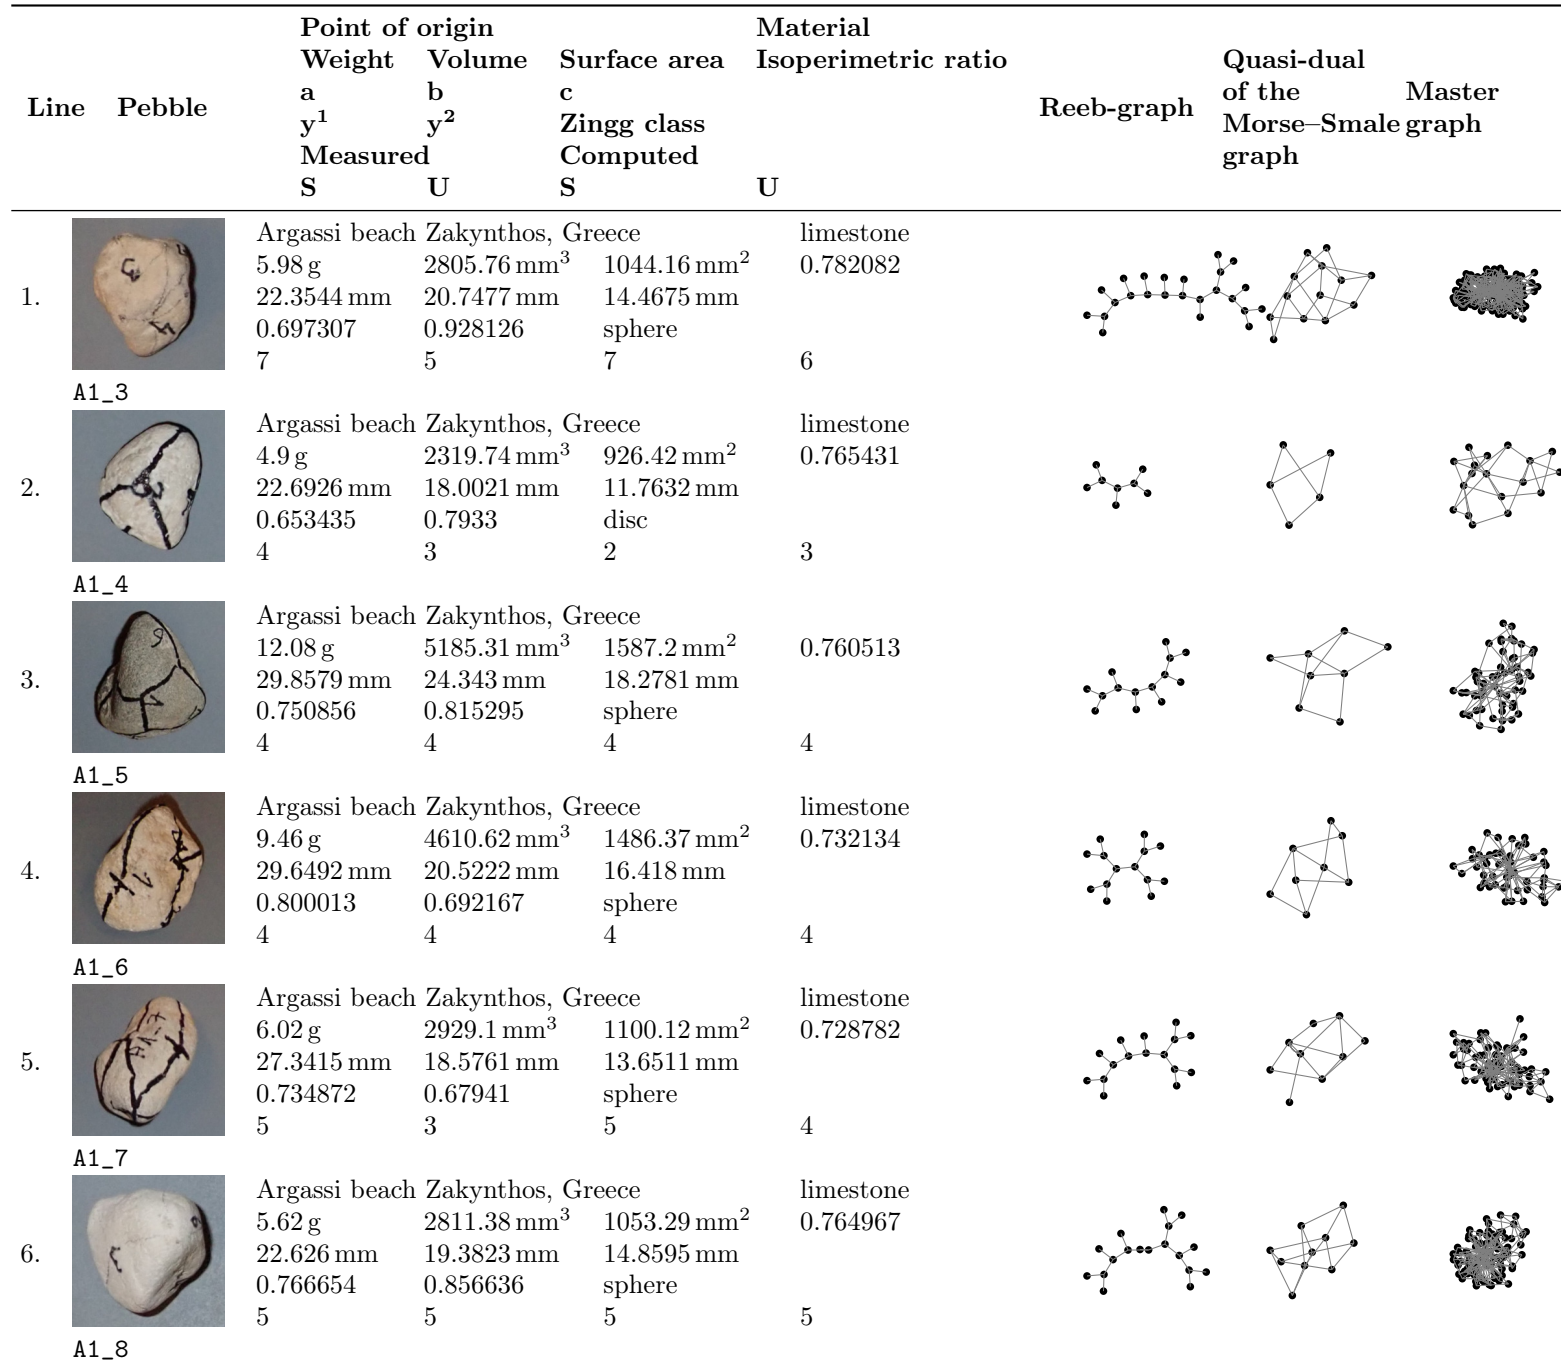   | 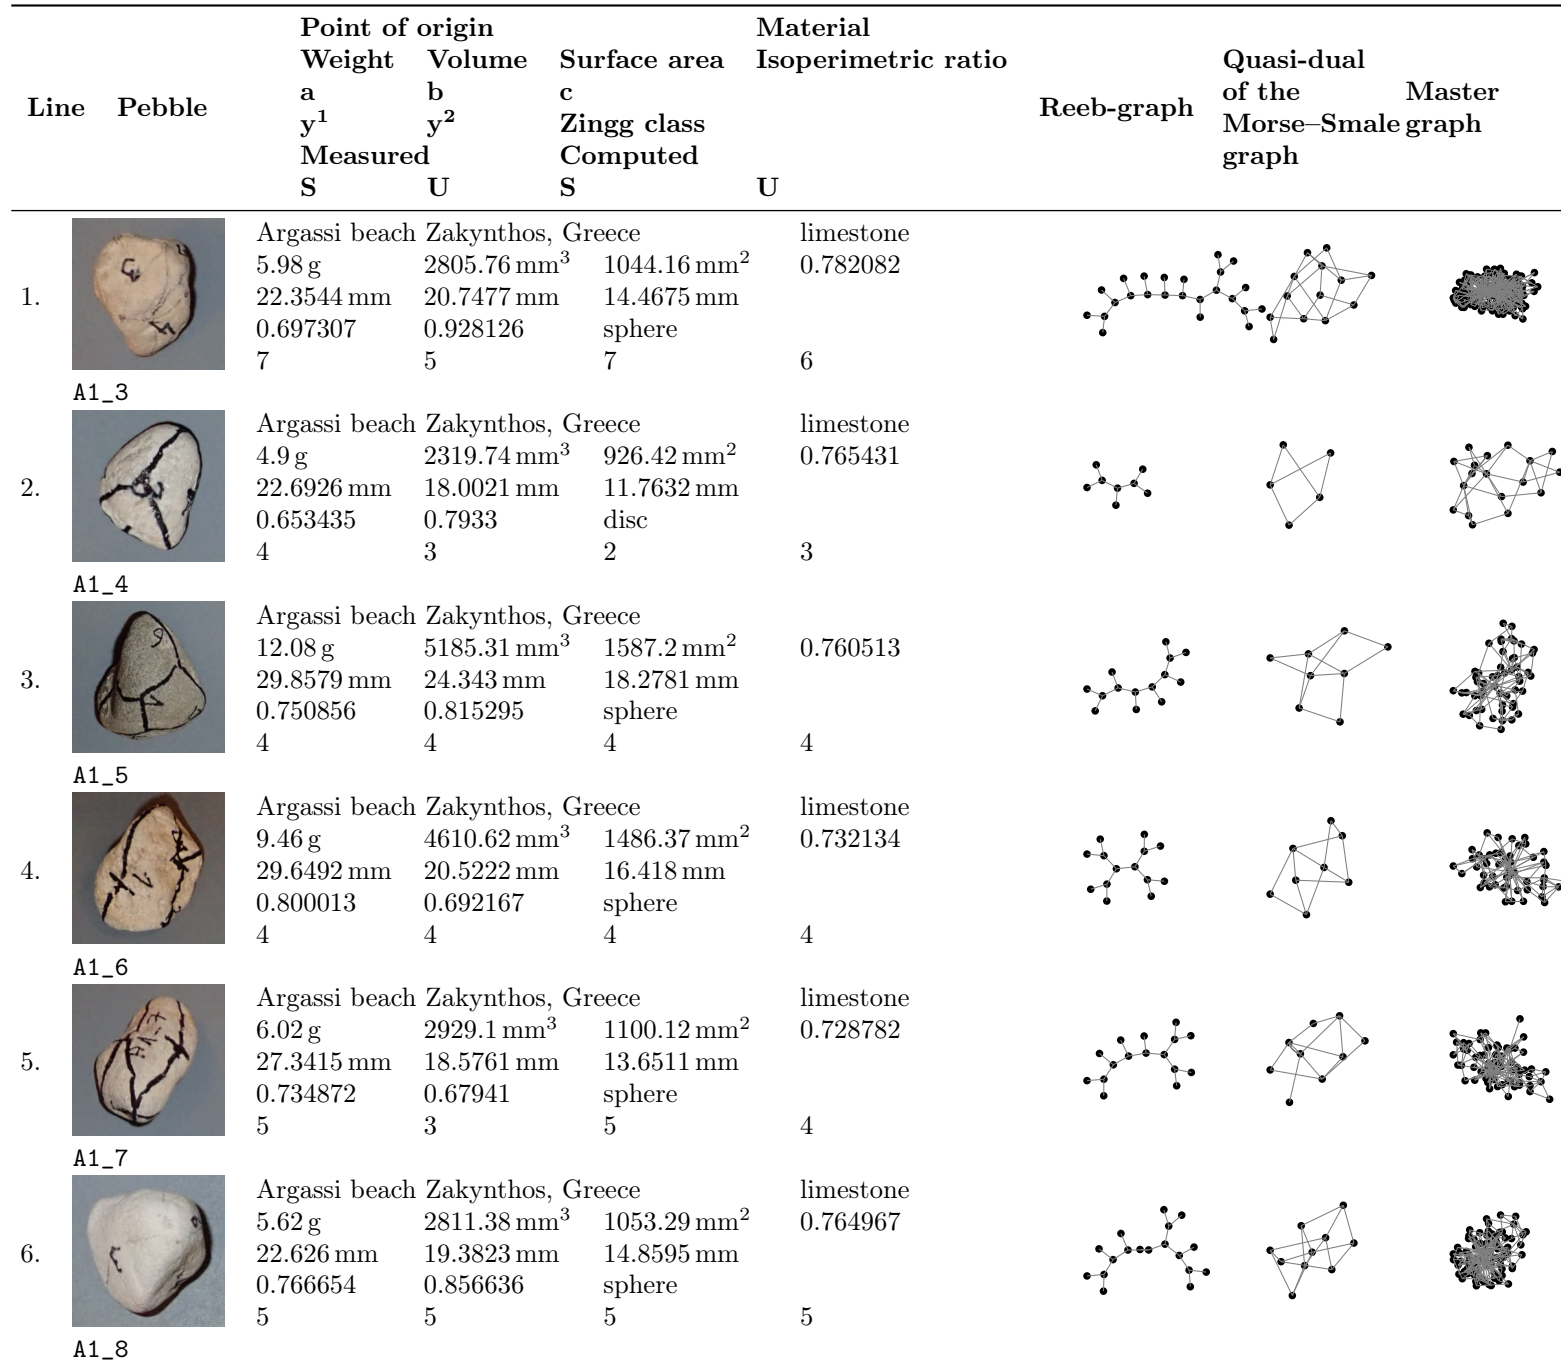   | 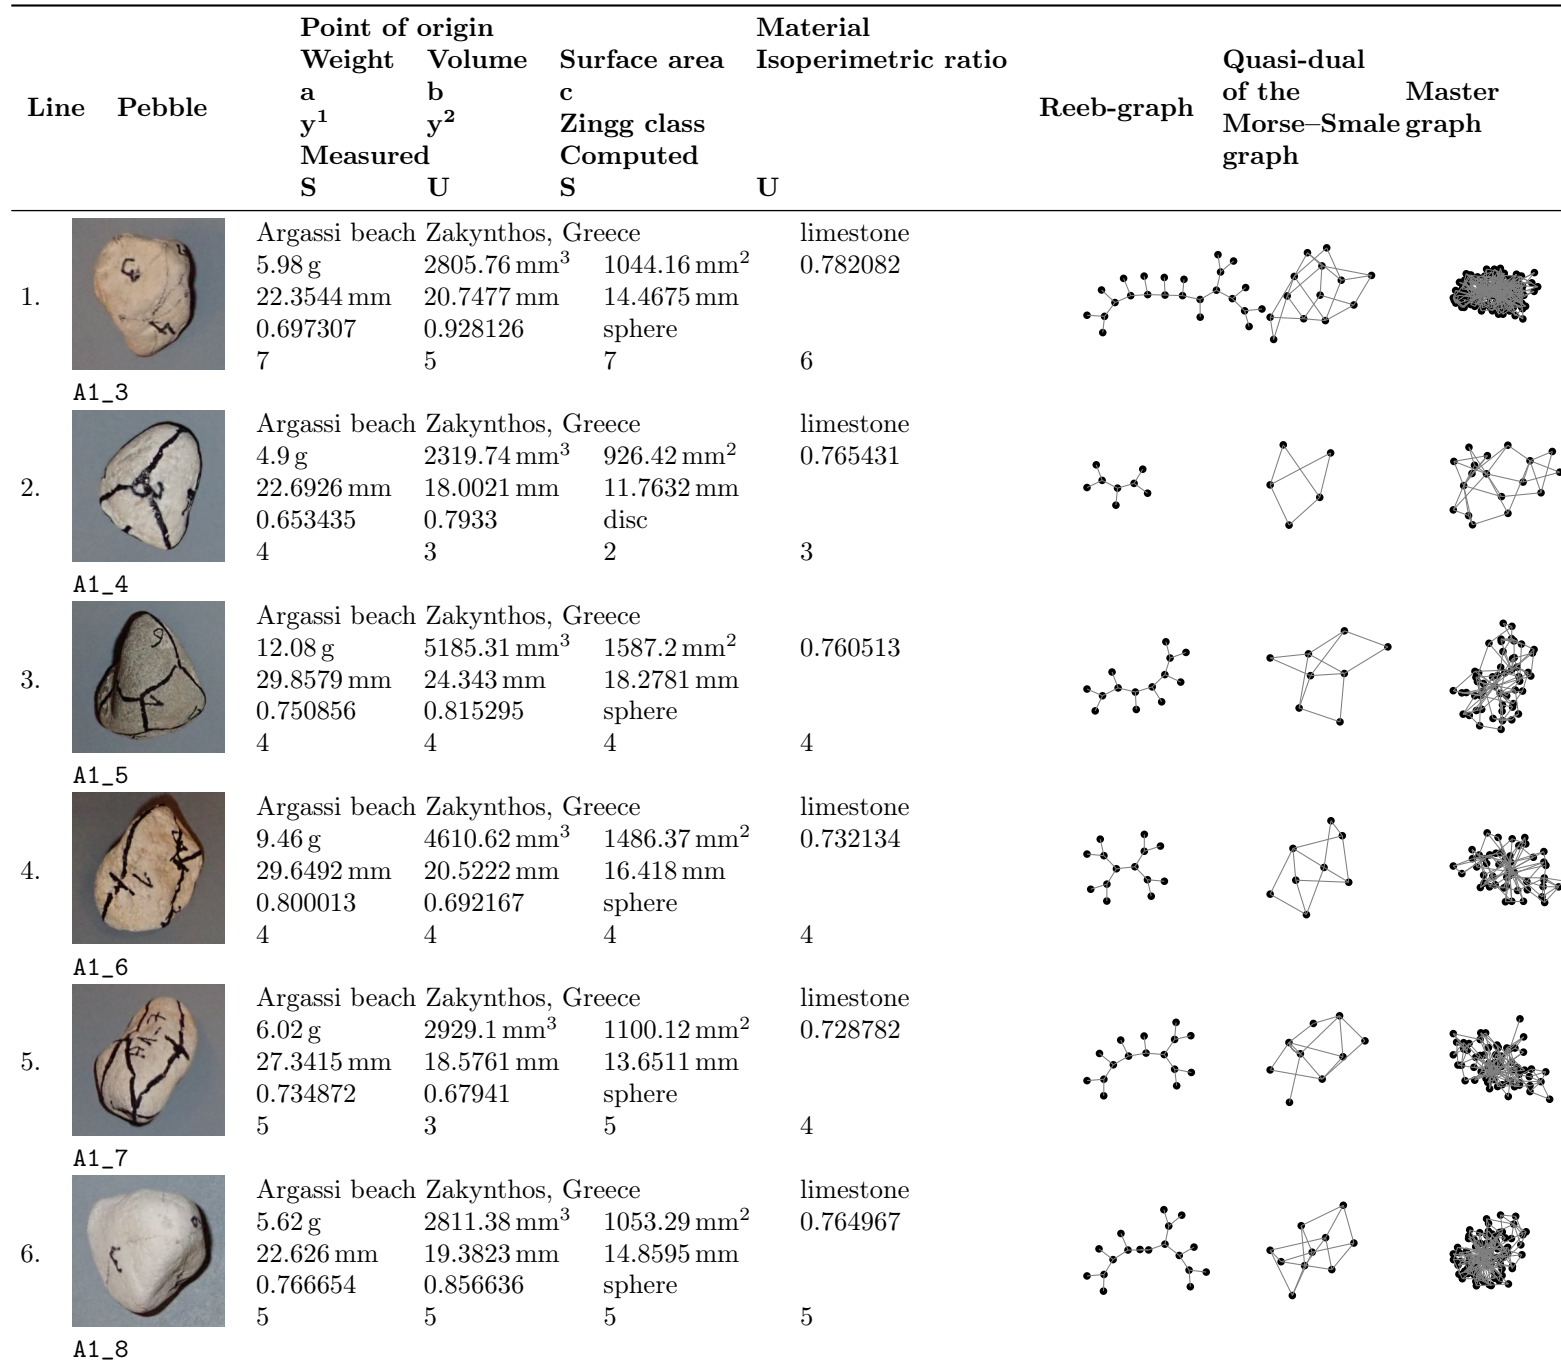   |
| A1_5 |                                                                                     |                                                         |                                                                             |                                                      |                                |                                                                                       |                                                                                       |                                                                                       |
| 4.   | 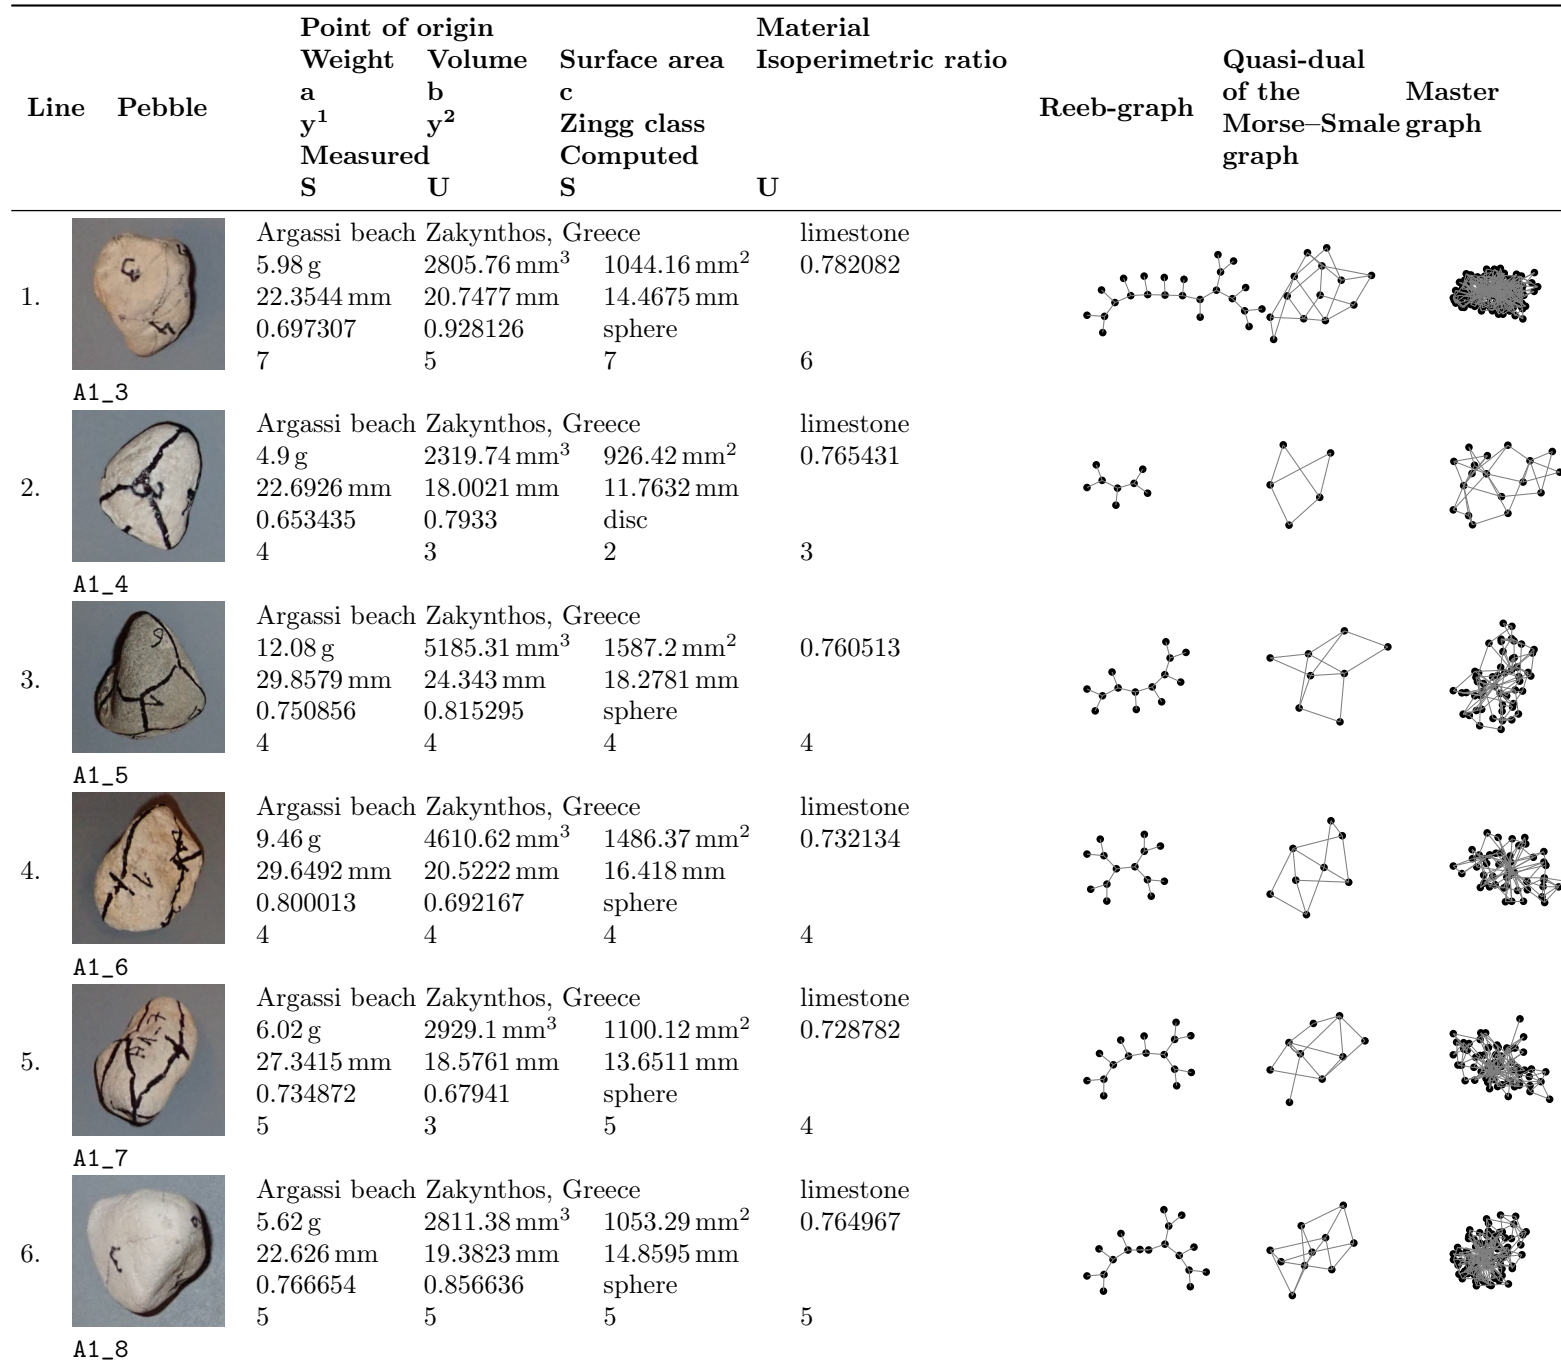  | Argassi beach<br>9.46 g<br>29.6492 mm<br>0.800013<br>4  | Zakynthos, Greece<br>4610.62 mm <sup>3</sup><br>20.5222 mm<br>0.692167<br>4 | 1486.37 mm <sup>2</sup><br>16.418 mm<br>sphere<br>4  | limestone<br>0.732134<br><br>4 | 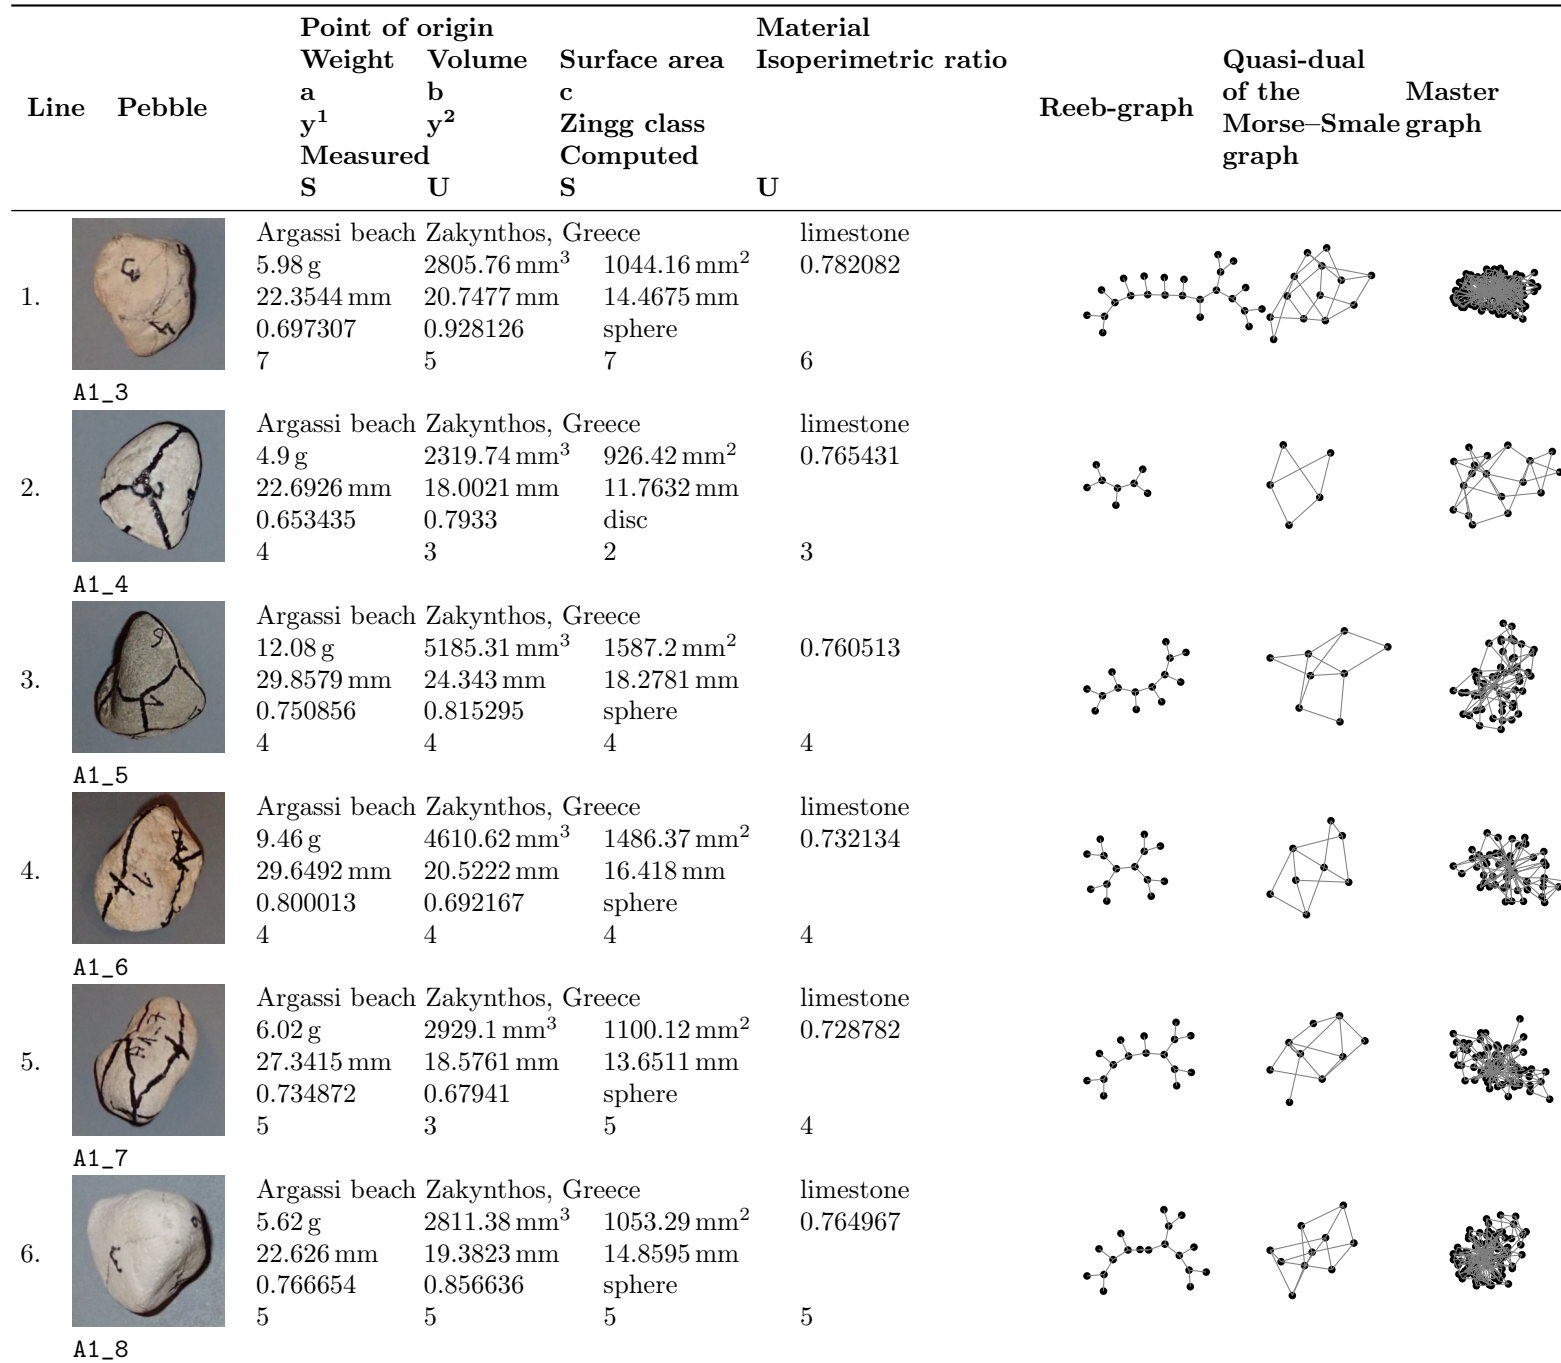  | 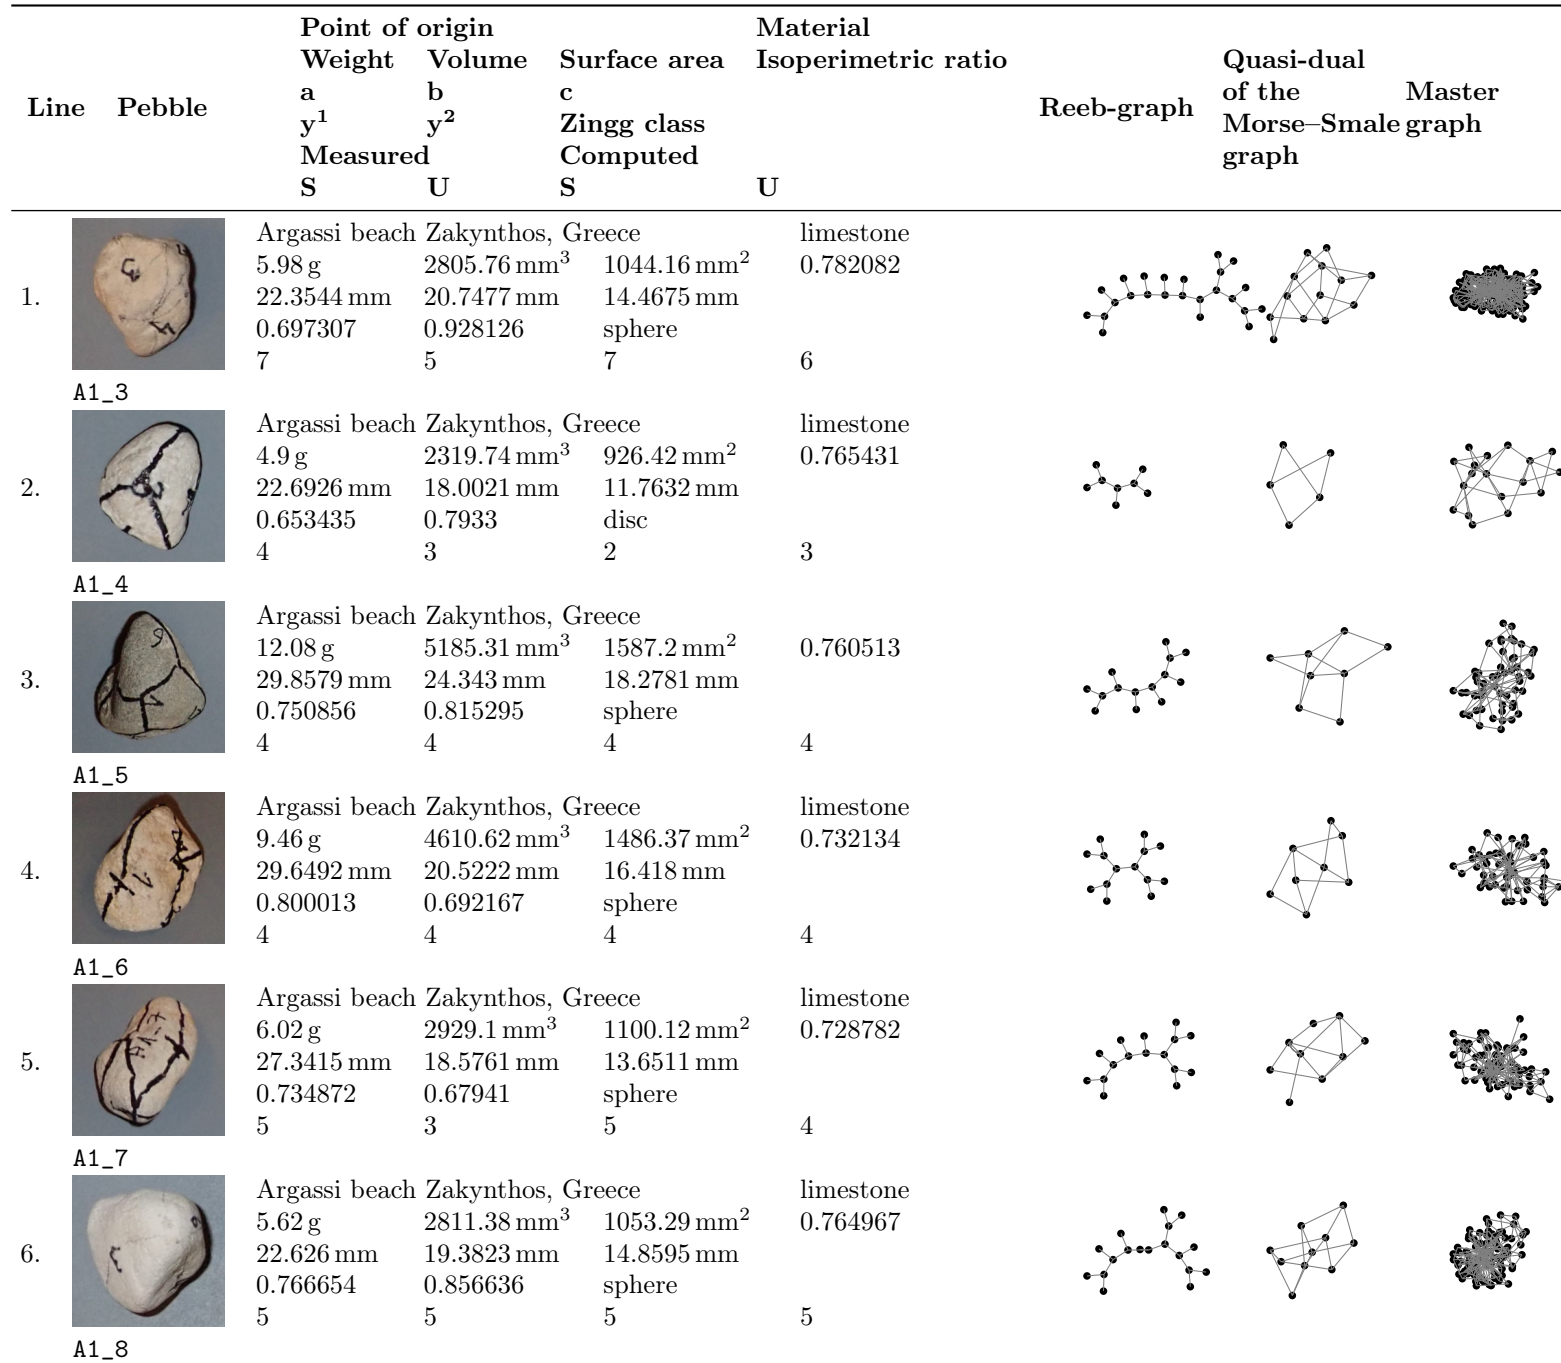  | 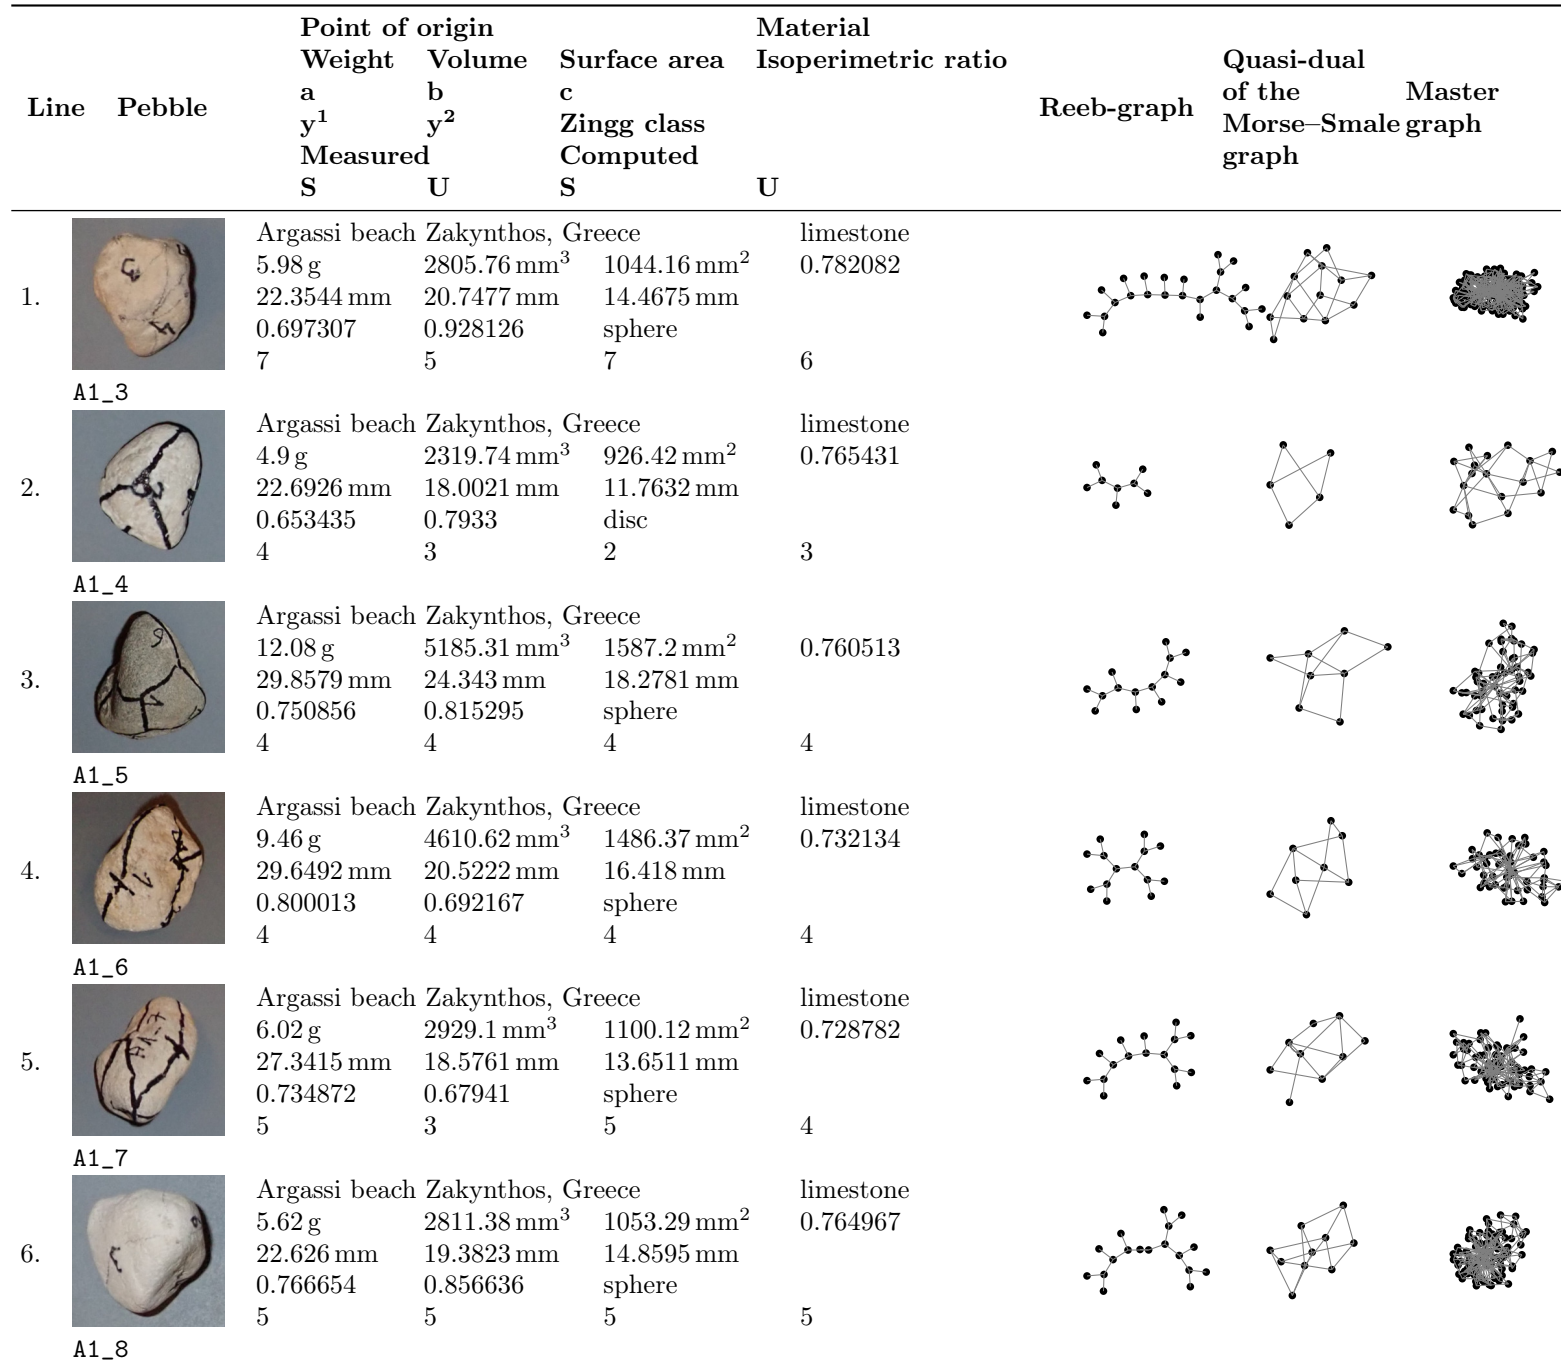  |
| A1_6 |                                                                                     |                                                         |                                                                             |                                                      |                                |                                                                                       |                                                                                       |                                                                                       |
| 5.   | 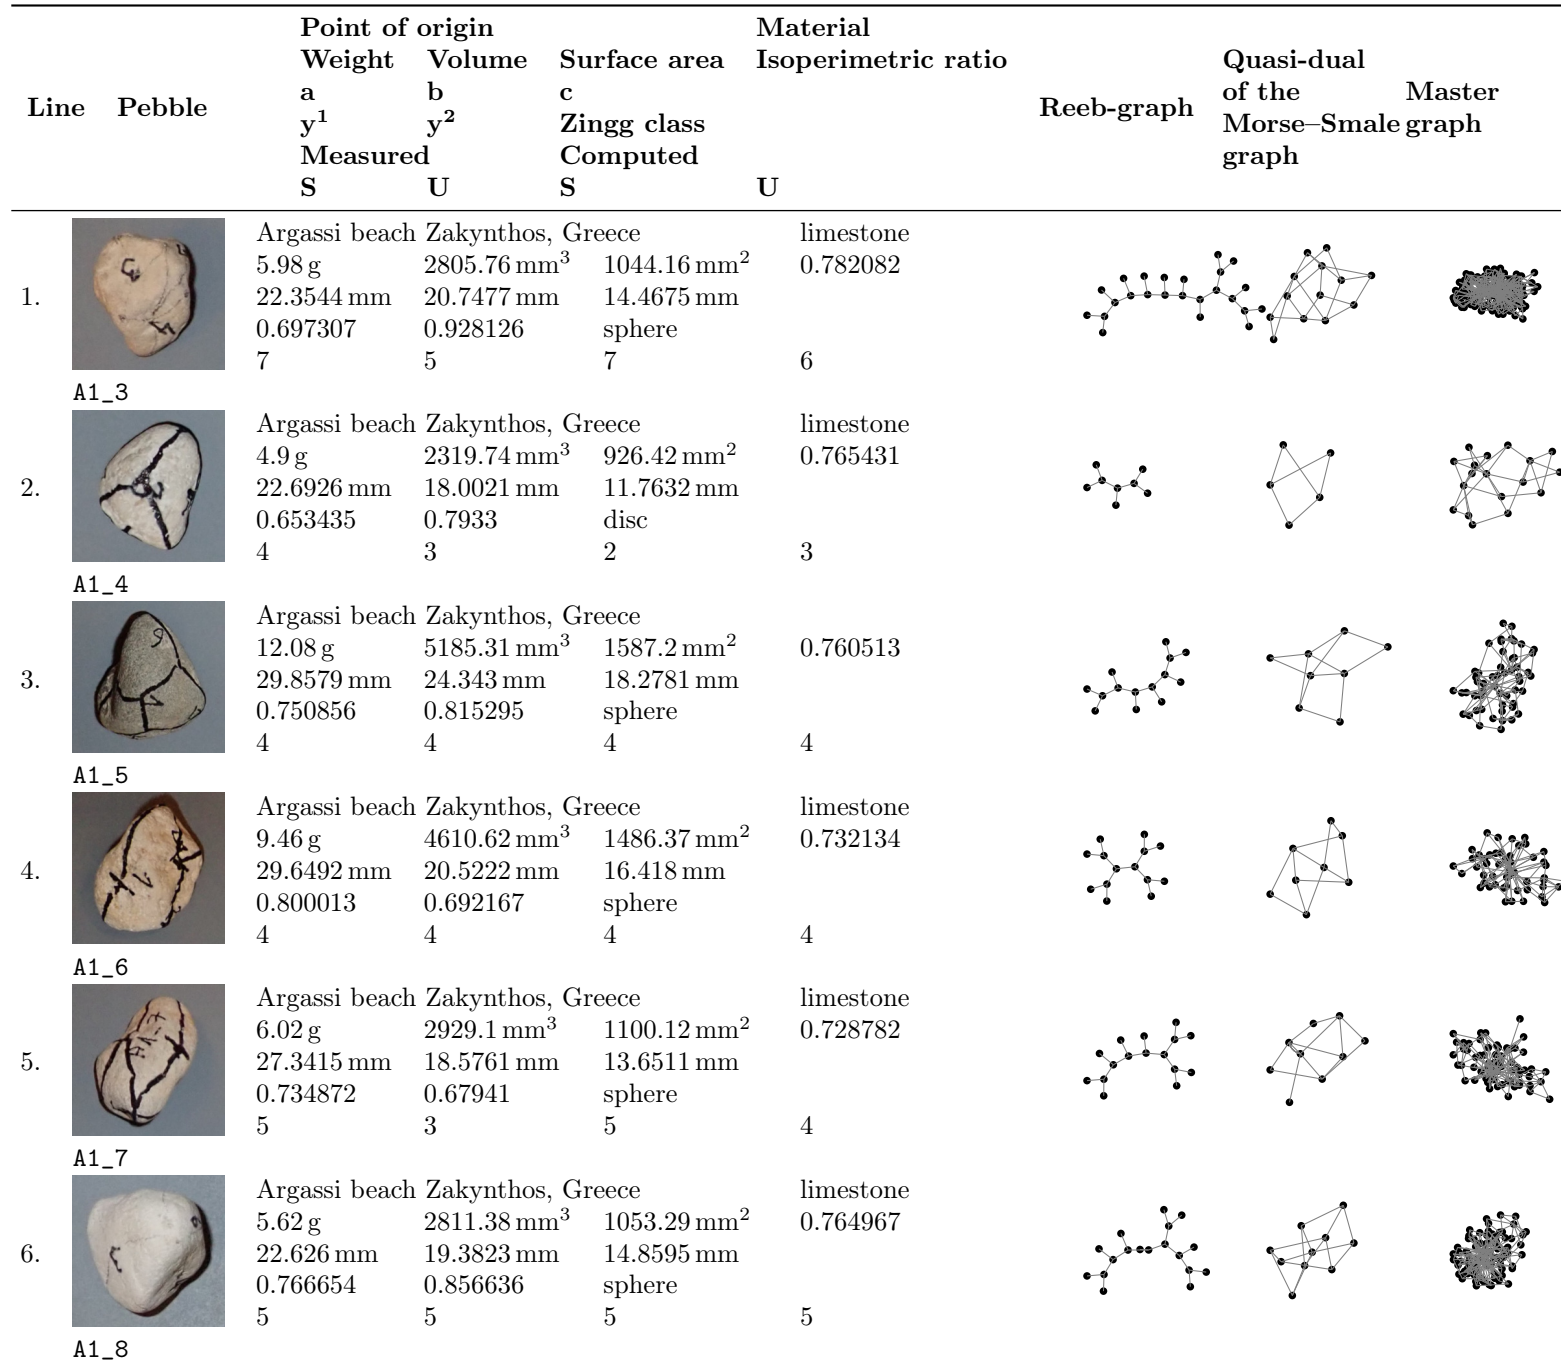 | Argassi beach<br>6.02 g<br>27.3415 mm<br>0.734872<br>5  | Zakynthos, Greece<br>2929.1 mm <sup>3</sup><br>18.5761 mm<br>0.67941<br>3   | 1100.12 mm <sup>2</sup><br>13.6511 mm<br>sphere<br>5 | limestone<br>0.728782<br><br>4 | 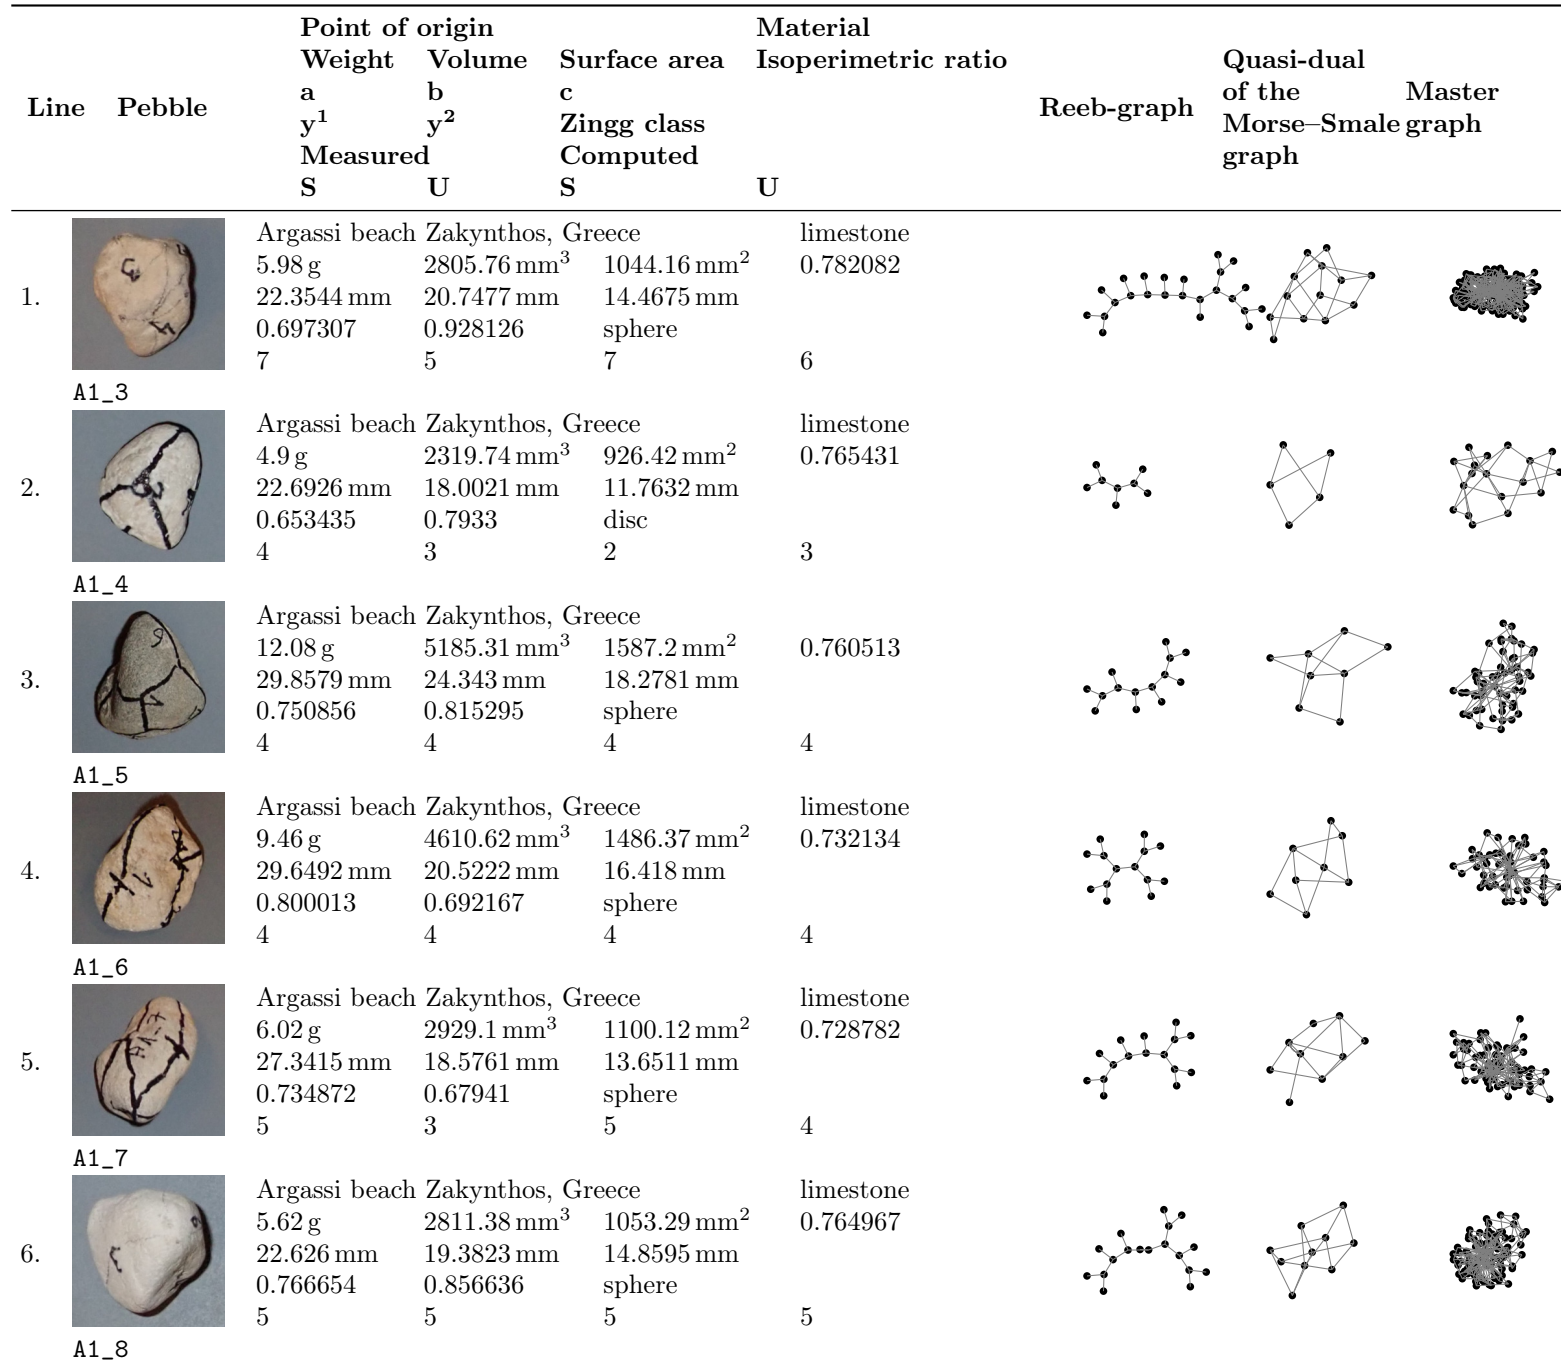 | 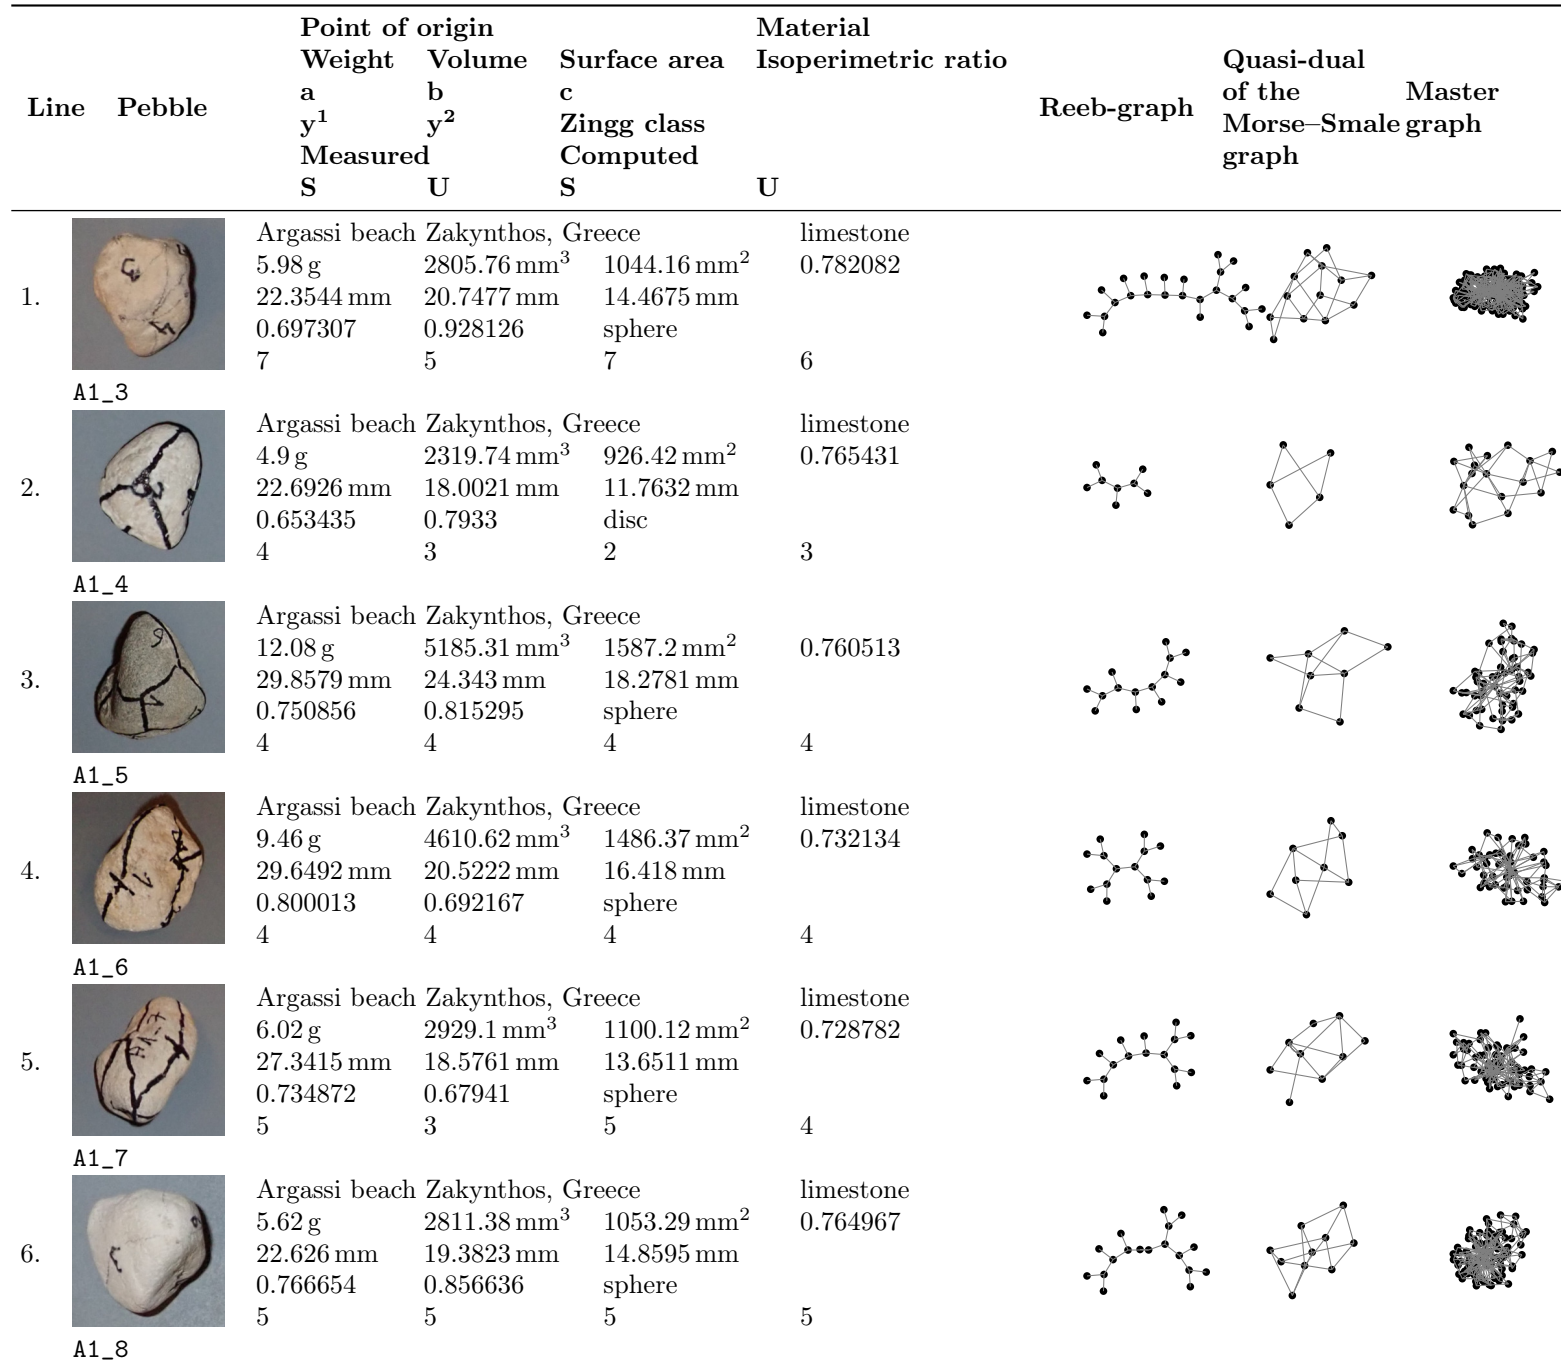 | 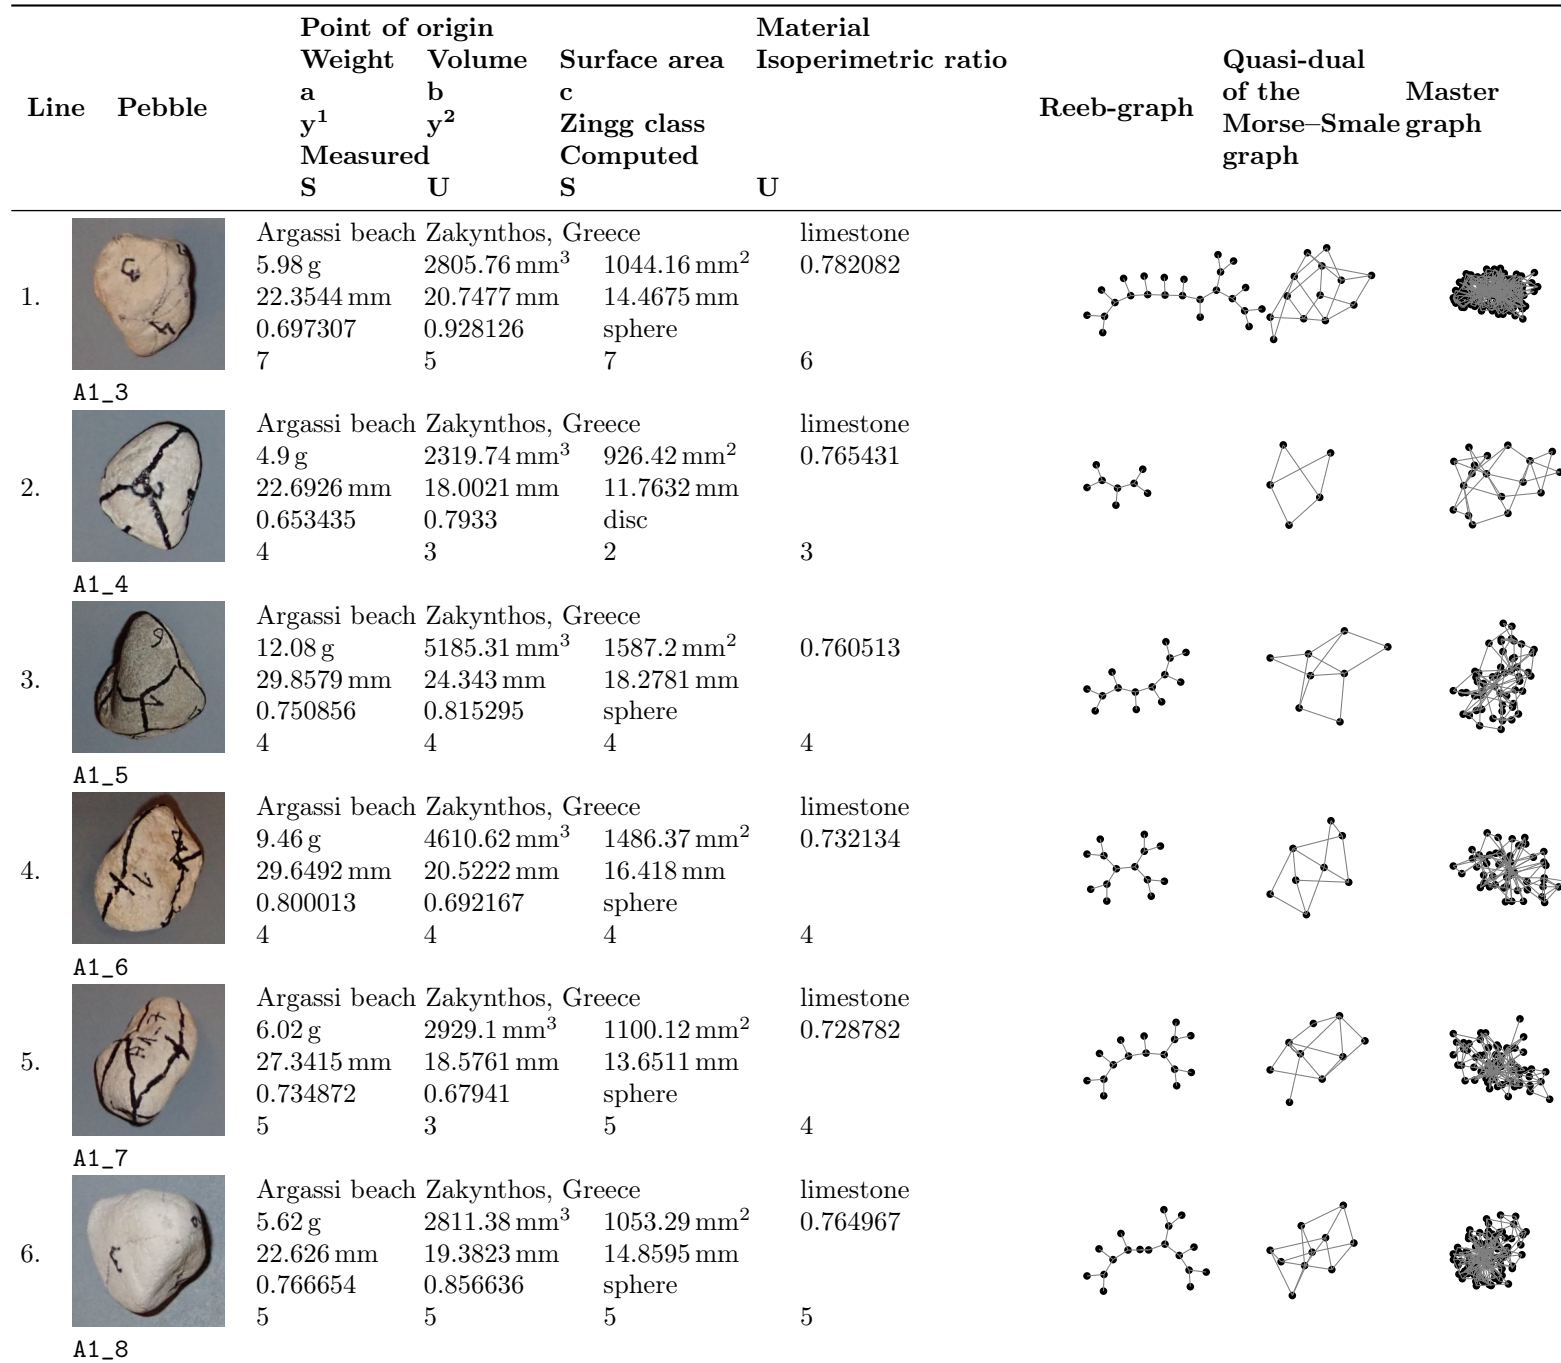 |
| A1_7 |                                                                                     |                                                         |                                                                             |                                                      |                                |                                                                                       |                                                                                       |                                                                                       |
| 6.   | 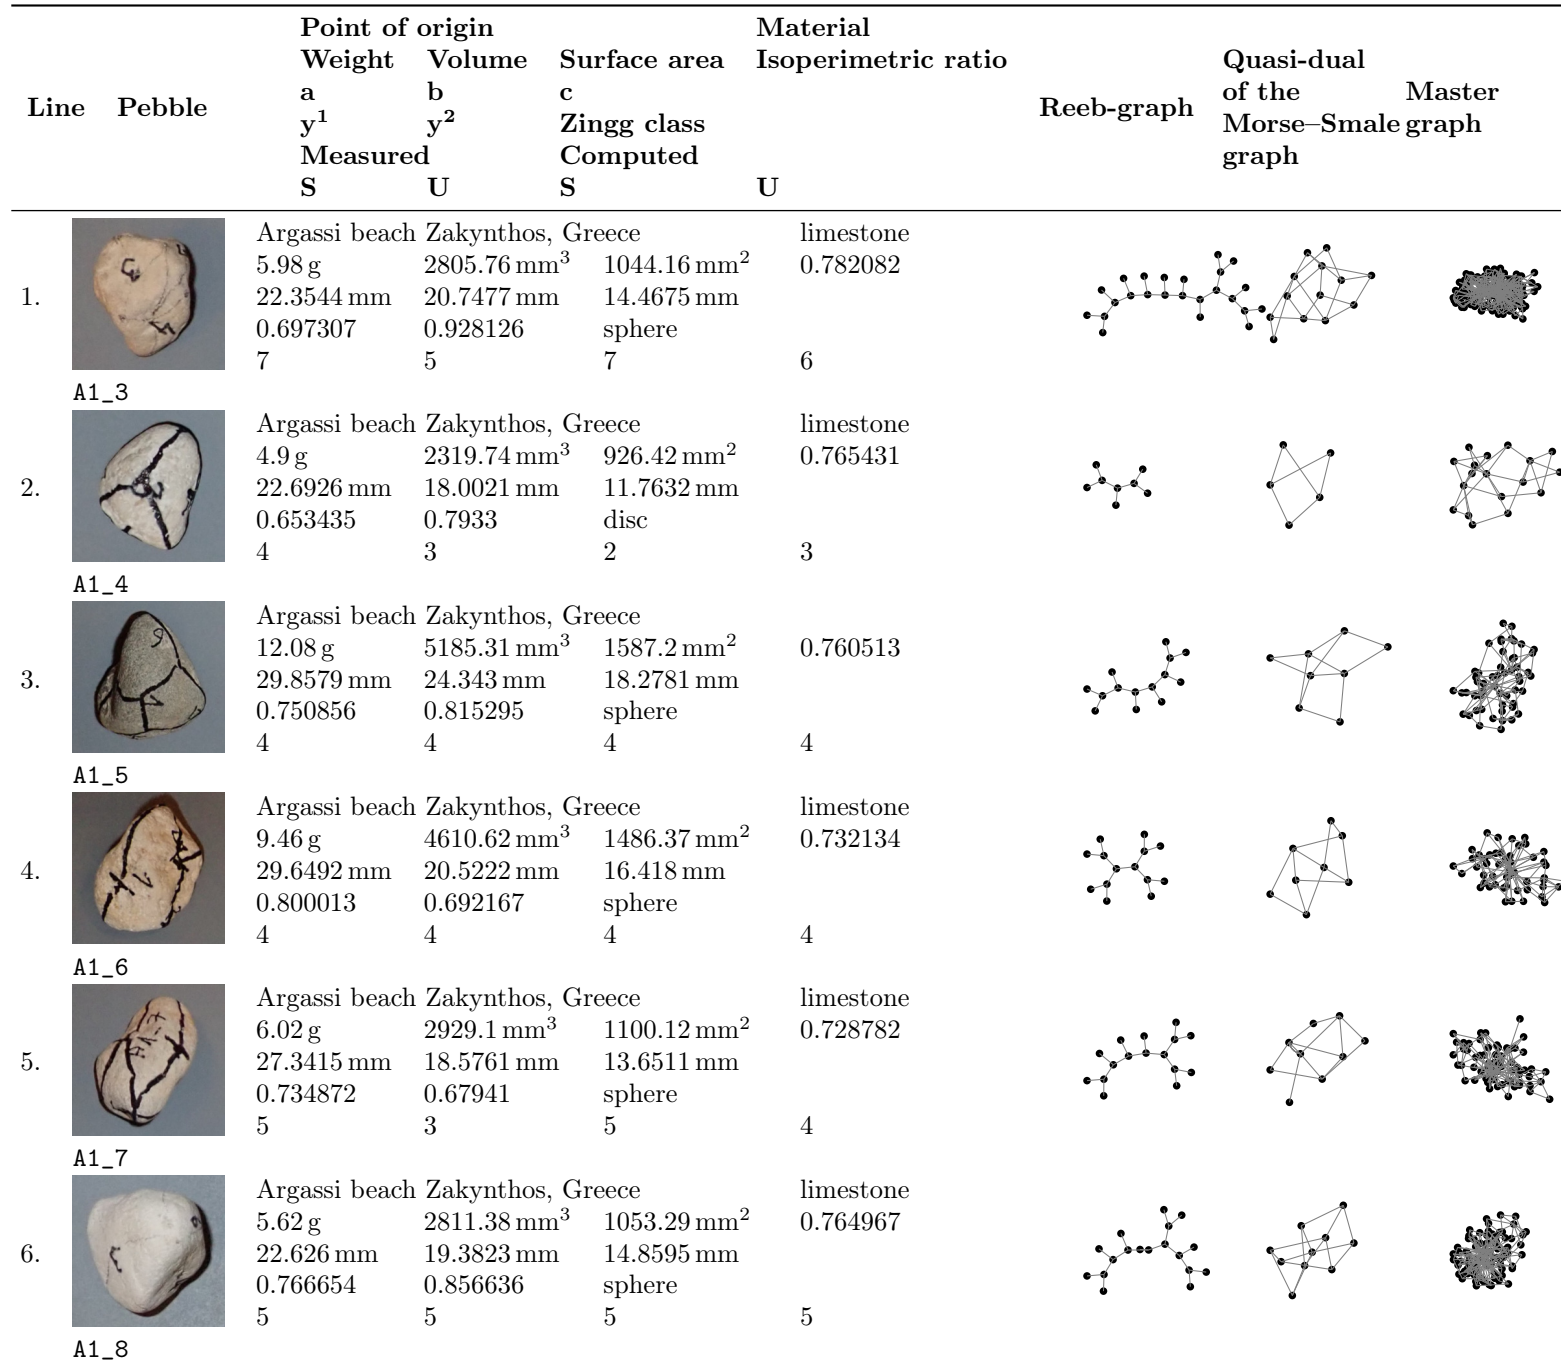 | Argassi beach<br>5.62 g<br>22.626 mm<br>0.766654<br>5   | Zakynthos, Greece<br>2811.38 mm <sup>3</sup><br>19.3823 mm<br>0.856636<br>5 | 1053.29 mm <sup>2</sup><br>14.8595 mm<br>sphere<br>5 | limestone<br>0.764967<br><br>5 | 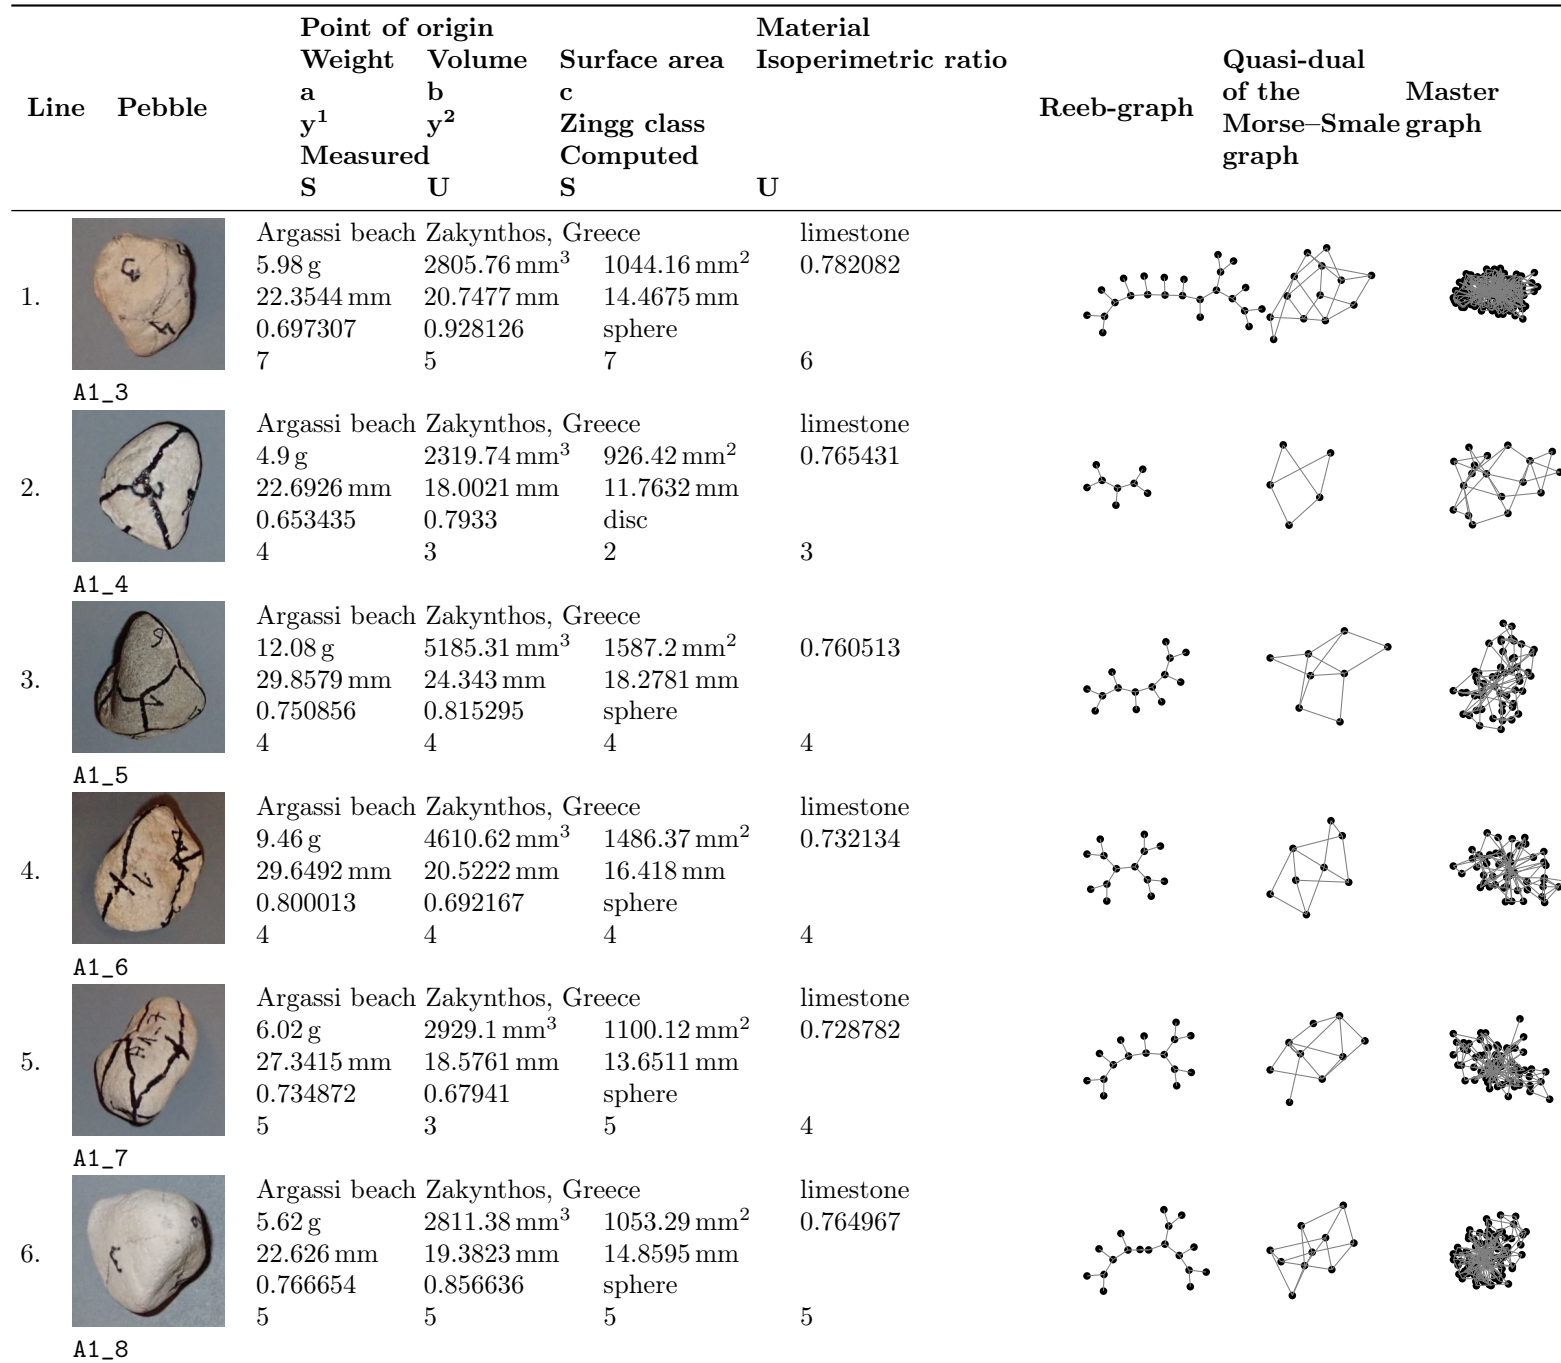 | 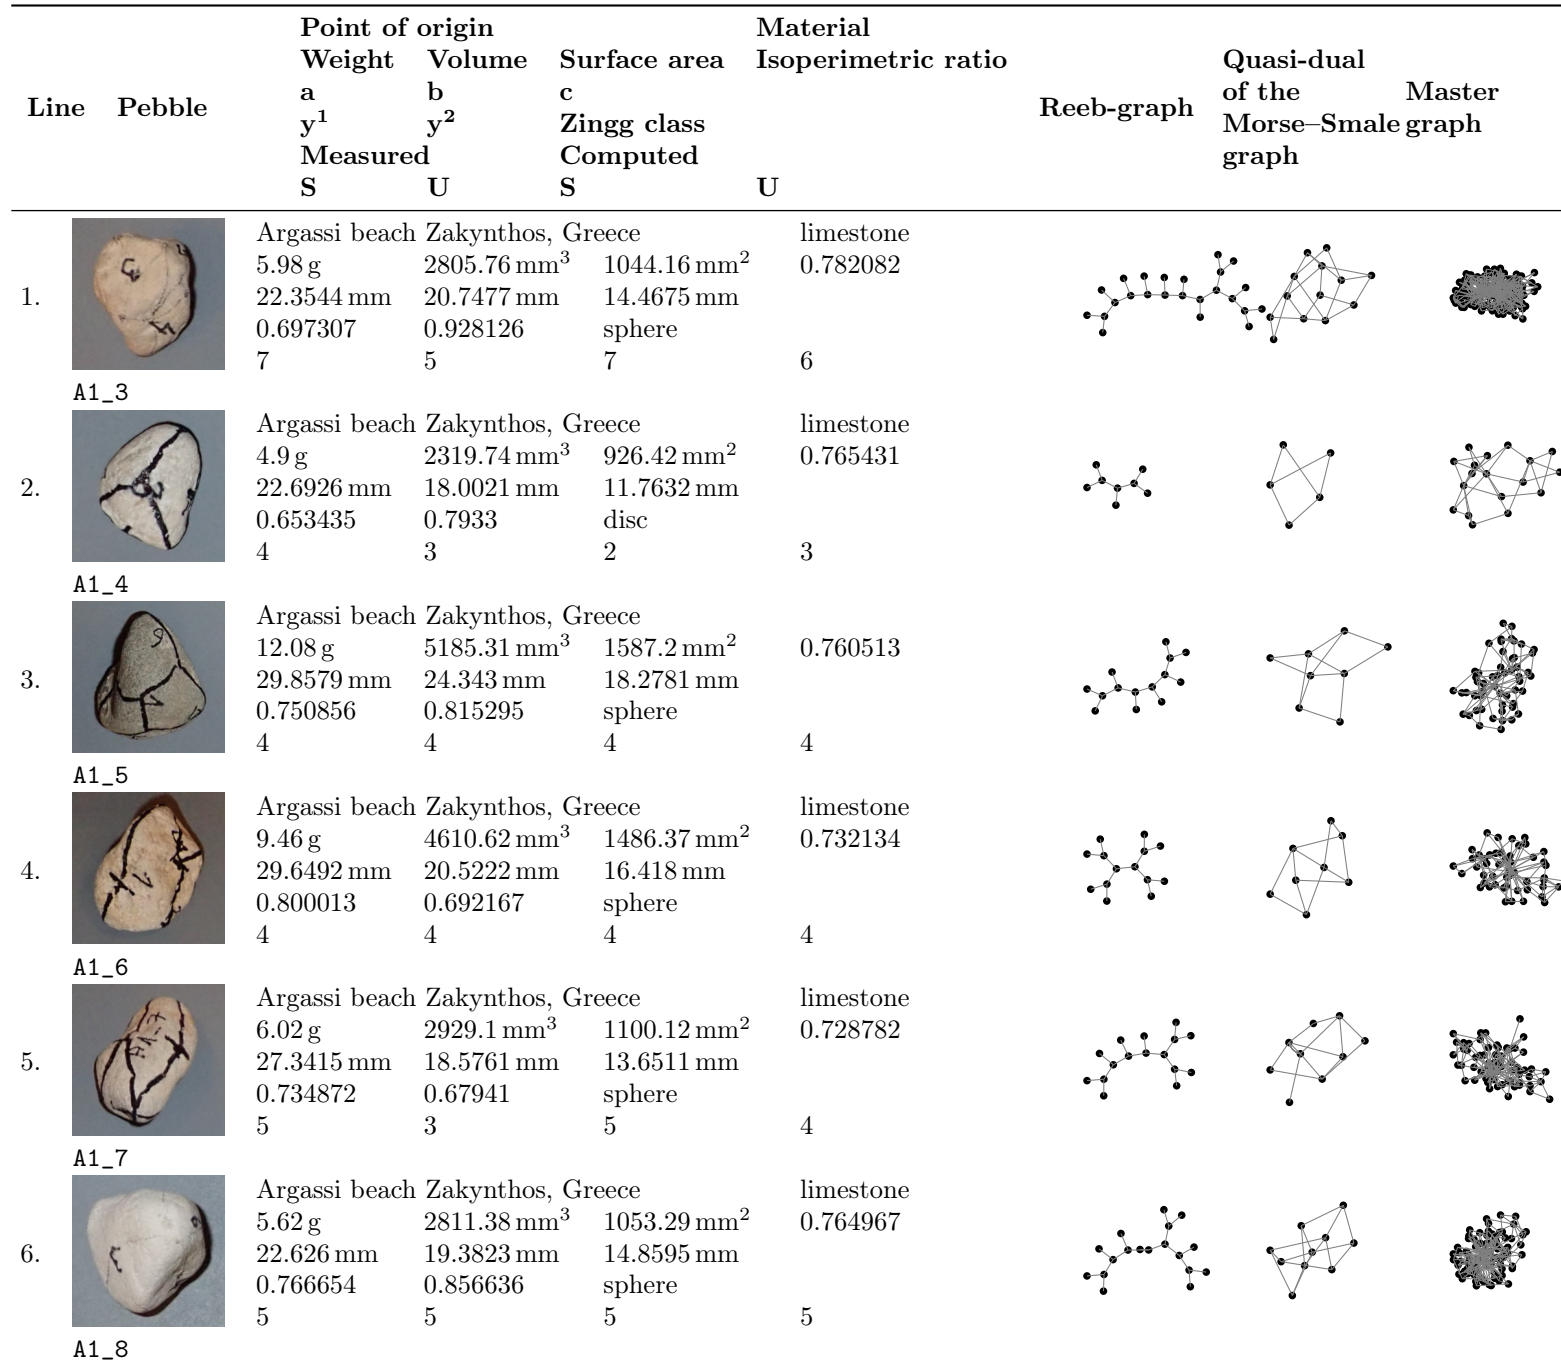 | 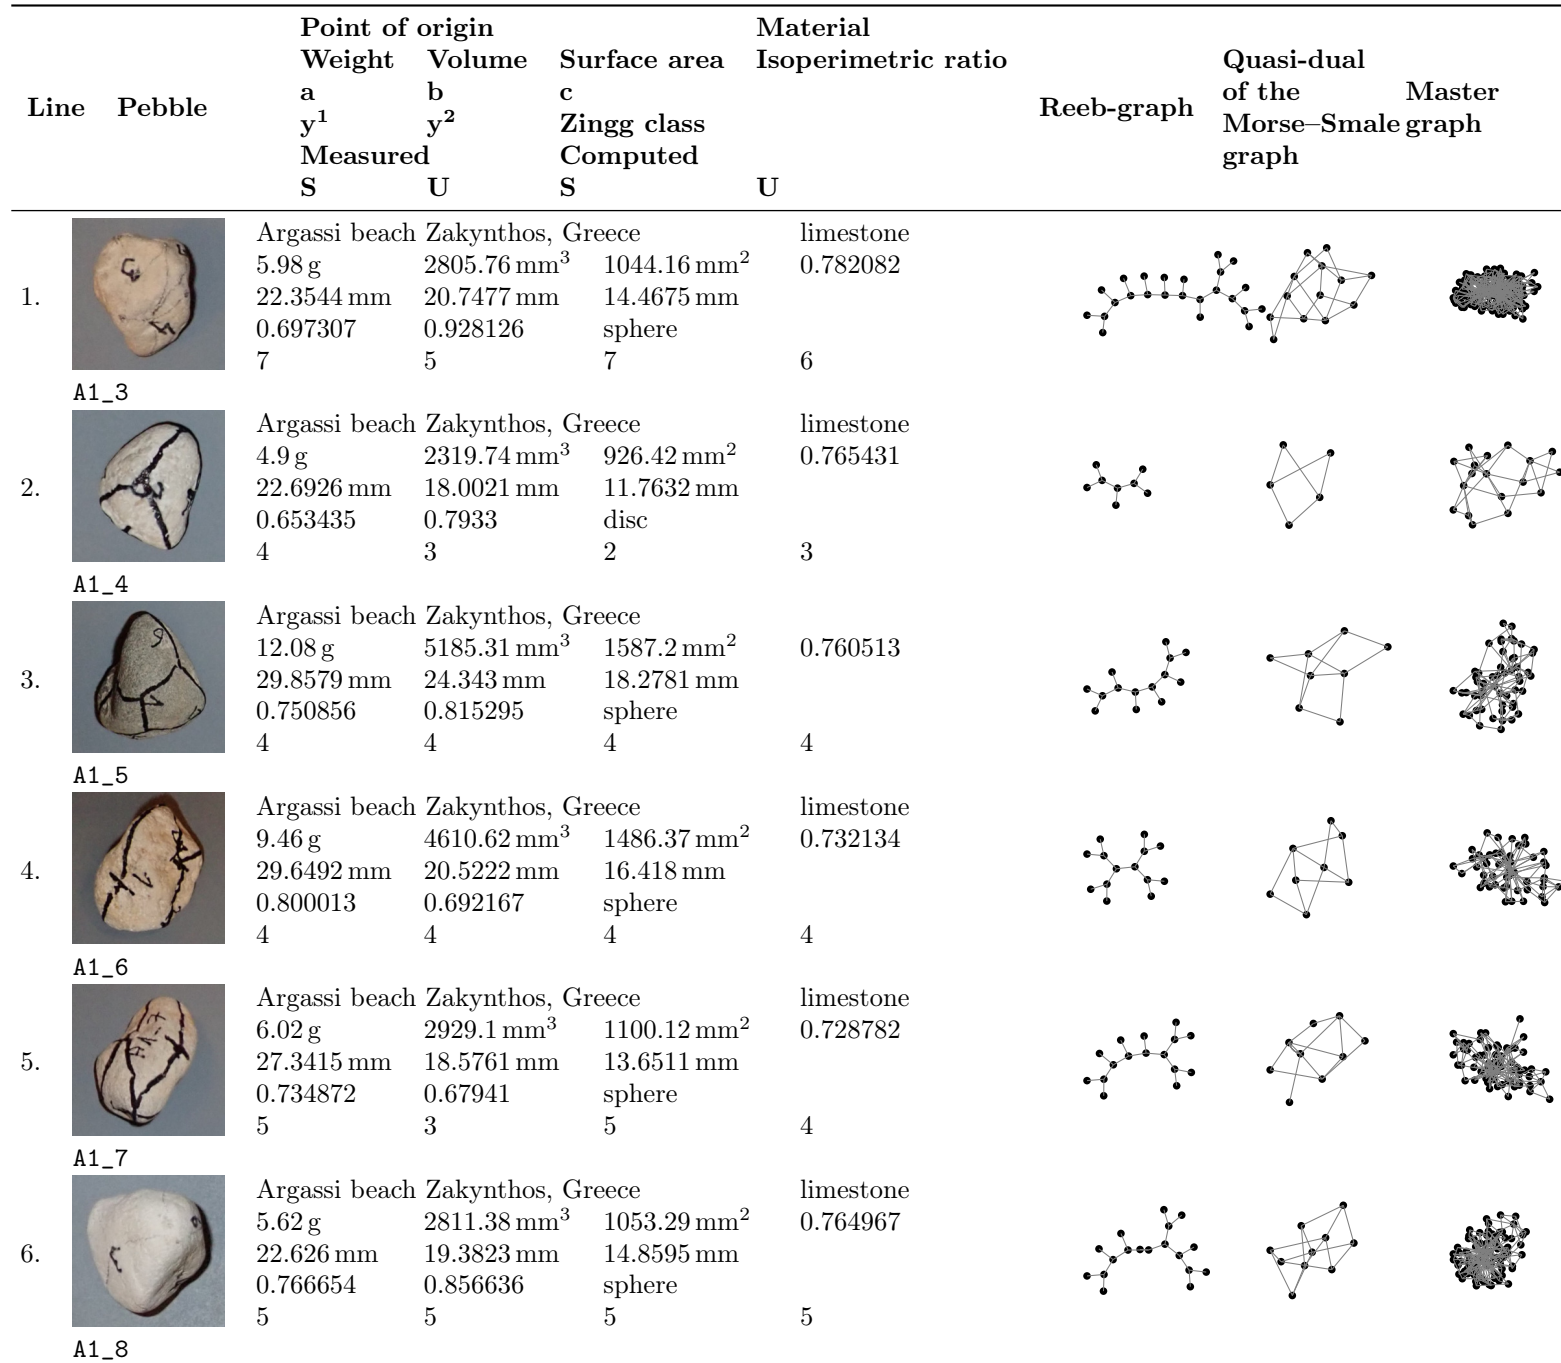 |
| A1_8 |                                                                                     |                                                         |                                                                             |                                                      |                                |                                                                                       |                                                                                       |                                                                                       |

| Line  | Pebble                                                                              | Point of origin                                        |                                                                             |                                                      | Material              | Reeb-graph                                                                            | Quasi-dual<br>of the<br>Morse–Smale<br>graph                                          | Master<br>graph                                                                       |
|-------|-------------------------------------------------------------------------------------|--------------------------------------------------------|-----------------------------------------------------------------------------|------------------------------------------------------|-----------------------|---------------------------------------------------------------------------------------|---------------------------------------------------------------------------------------|---------------------------------------------------------------------------------------|
|       |                                                                                     | Weight                                                 | Volume                                                                      | Surface area                                         |                       |                                                                                       |                                                                                       |                                                                                       |
|       |                                                                                     | a                                                      | b                                                                           | c                                                    |                       |                                                                                       |                                                                                       |                                                                                       |
|       |                                                                                     | y <sup>1</sup><br>Measured<br>S                        | y <sup>2</sup><br>U                                                         | Zingg class<br>Computed<br>S                         |                       |                                                                                       |                                                                                       |                                                                                       |
| 7.    | 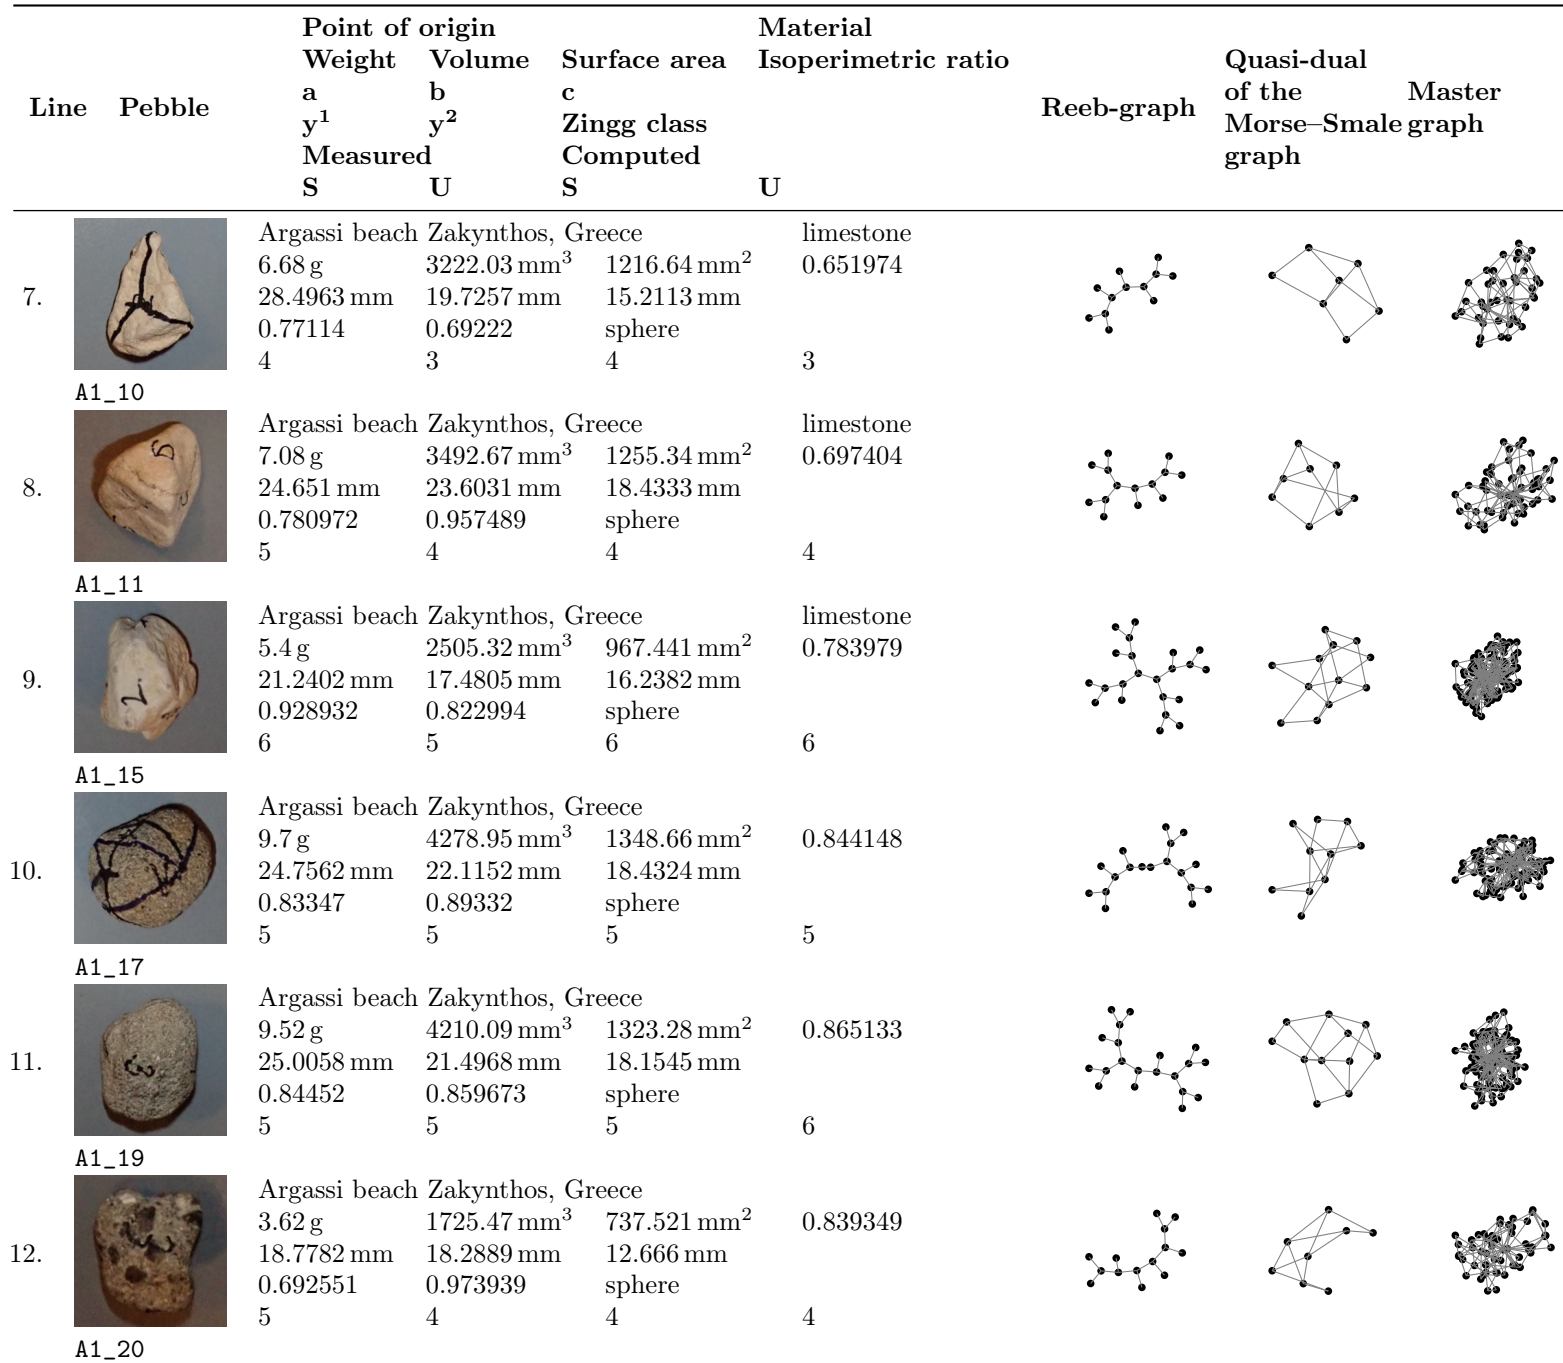   | Argassi beach<br>6.68 g<br>28.4963 mm<br>0.77114<br>4  | Zakynthos, Greece<br>3222.03 mm <sup>3</sup><br>19.7257 mm<br>0.69222<br>3  | 1216.64 mm <sup>2</sup><br>15.2113 mm<br>sphere<br>4 | limestone<br>0.651974 | 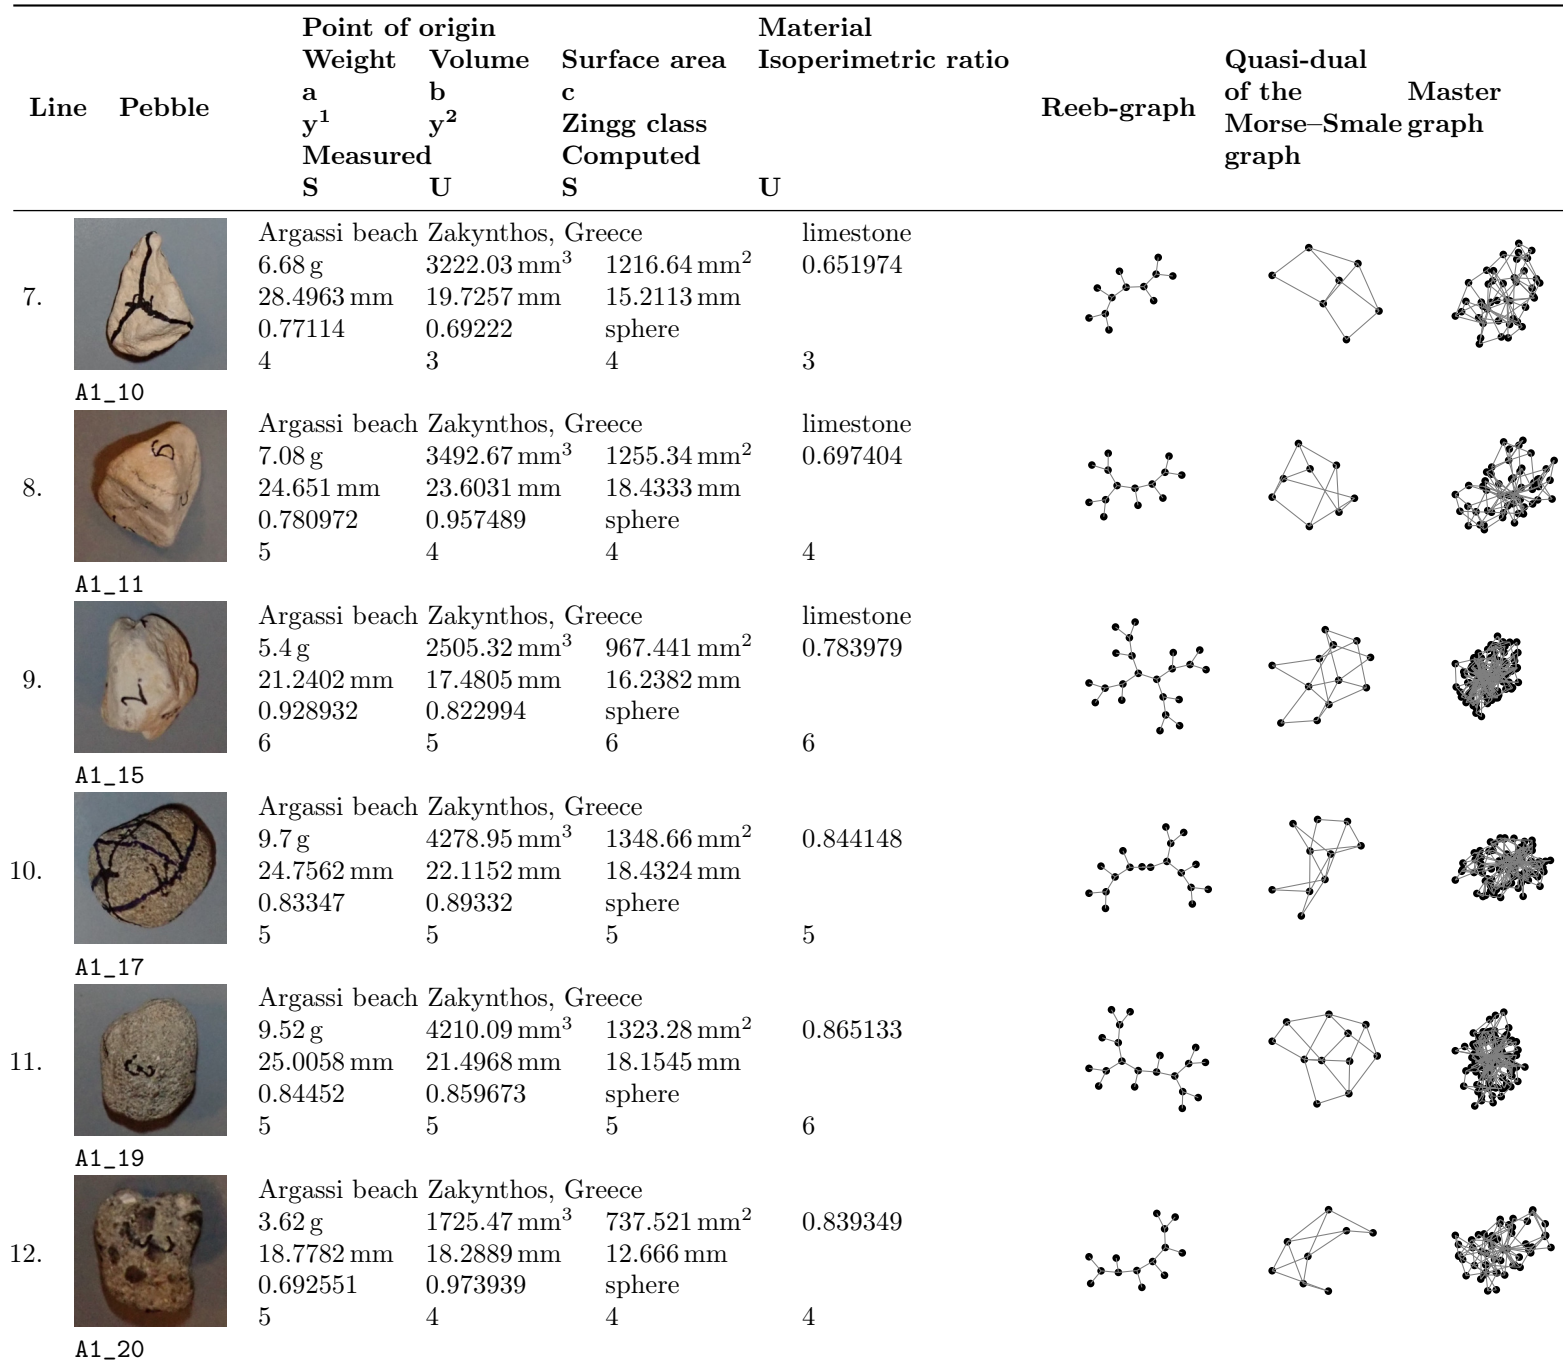   | 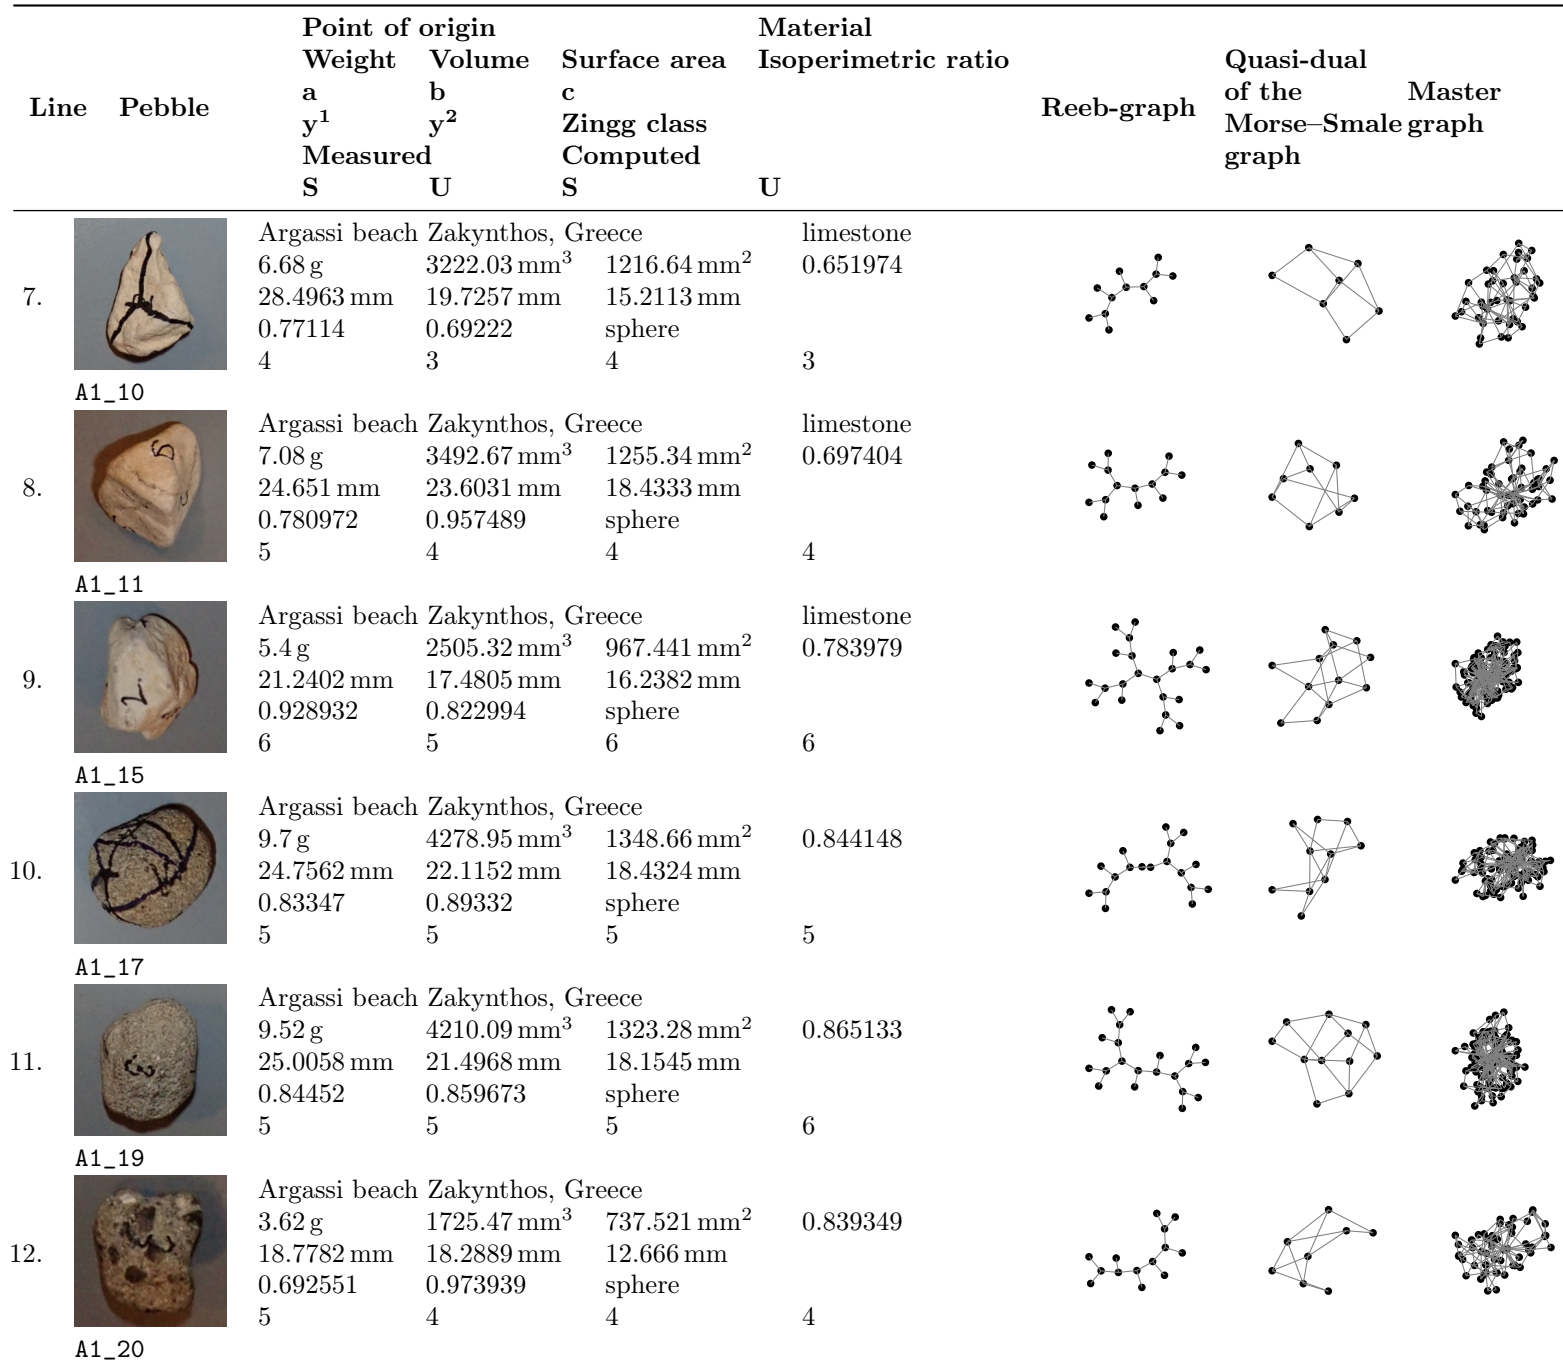   | 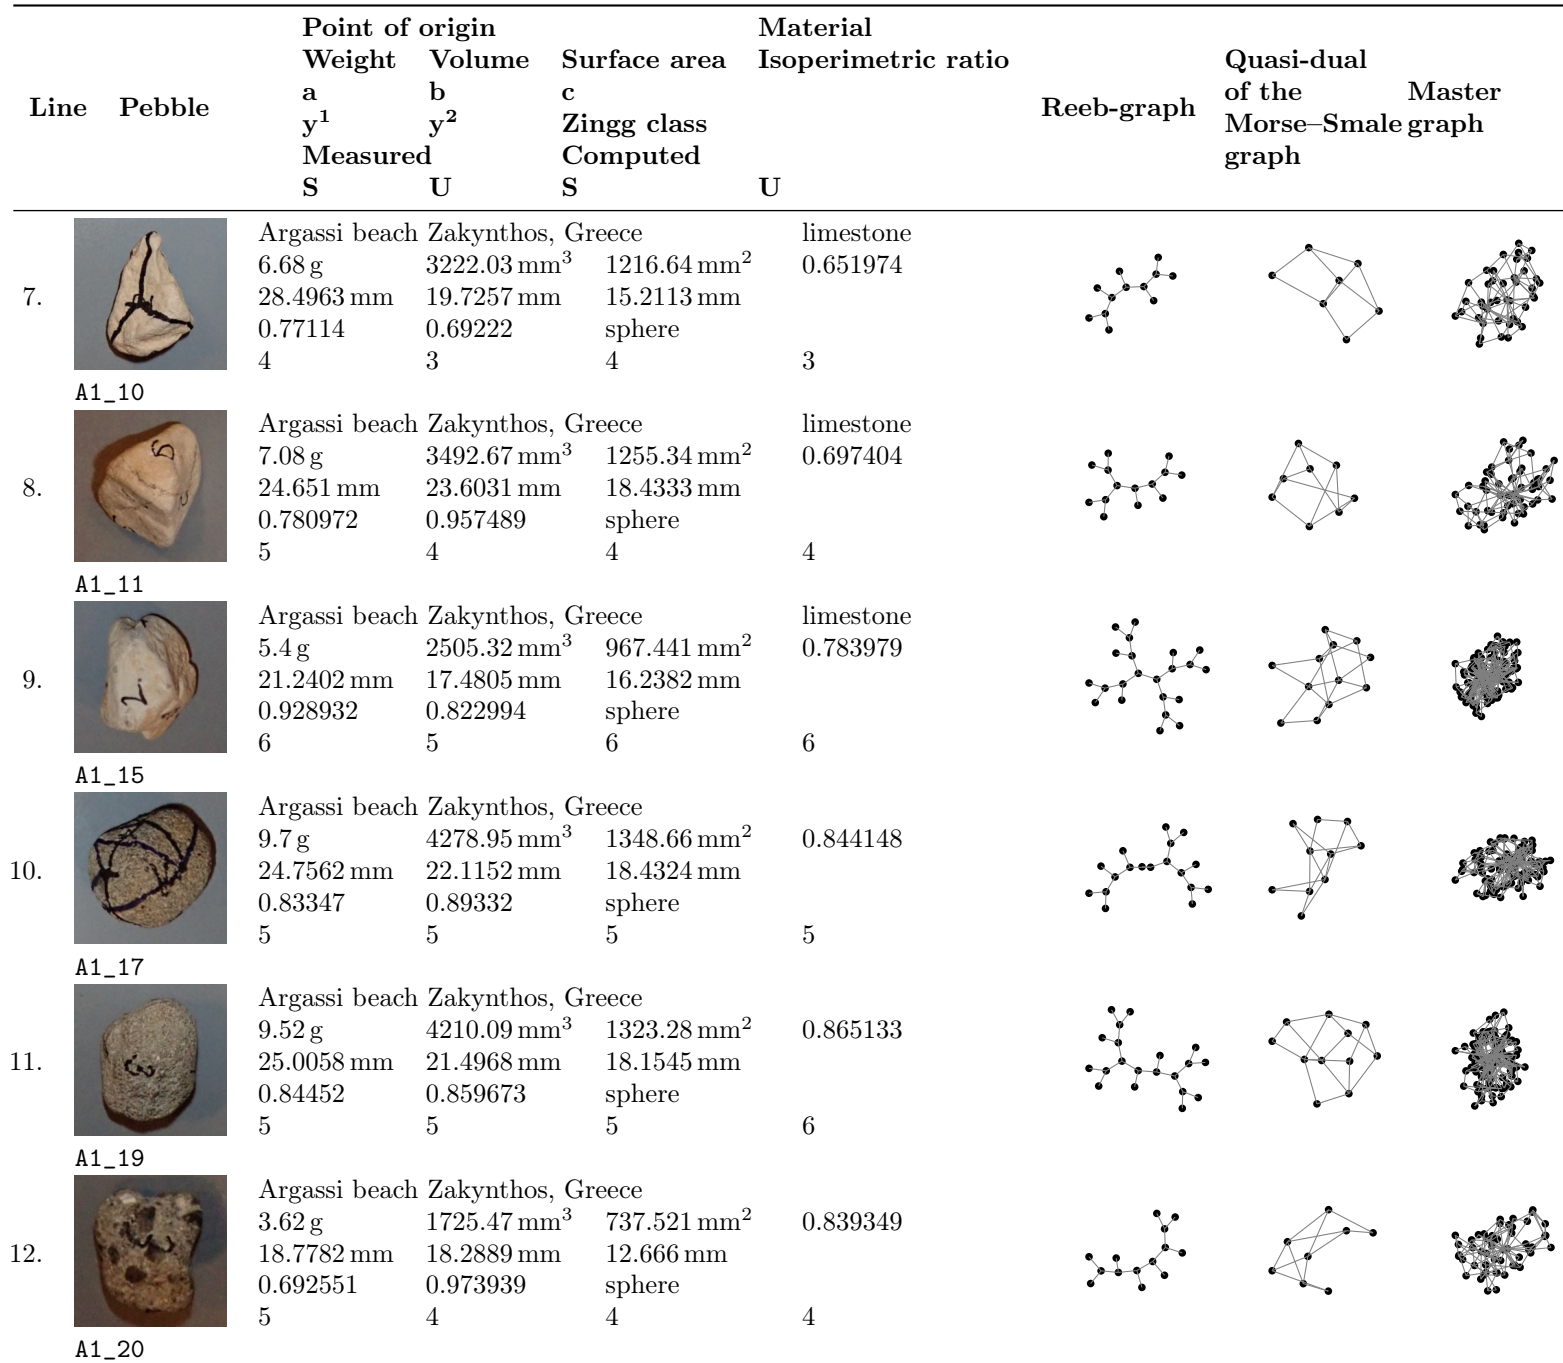   |
| A1_10 |                                                                                     |                                                        |                                                                             |                                                      |                       |                                                                                       |                                                                                       |                                                                                       |
| 8.    | 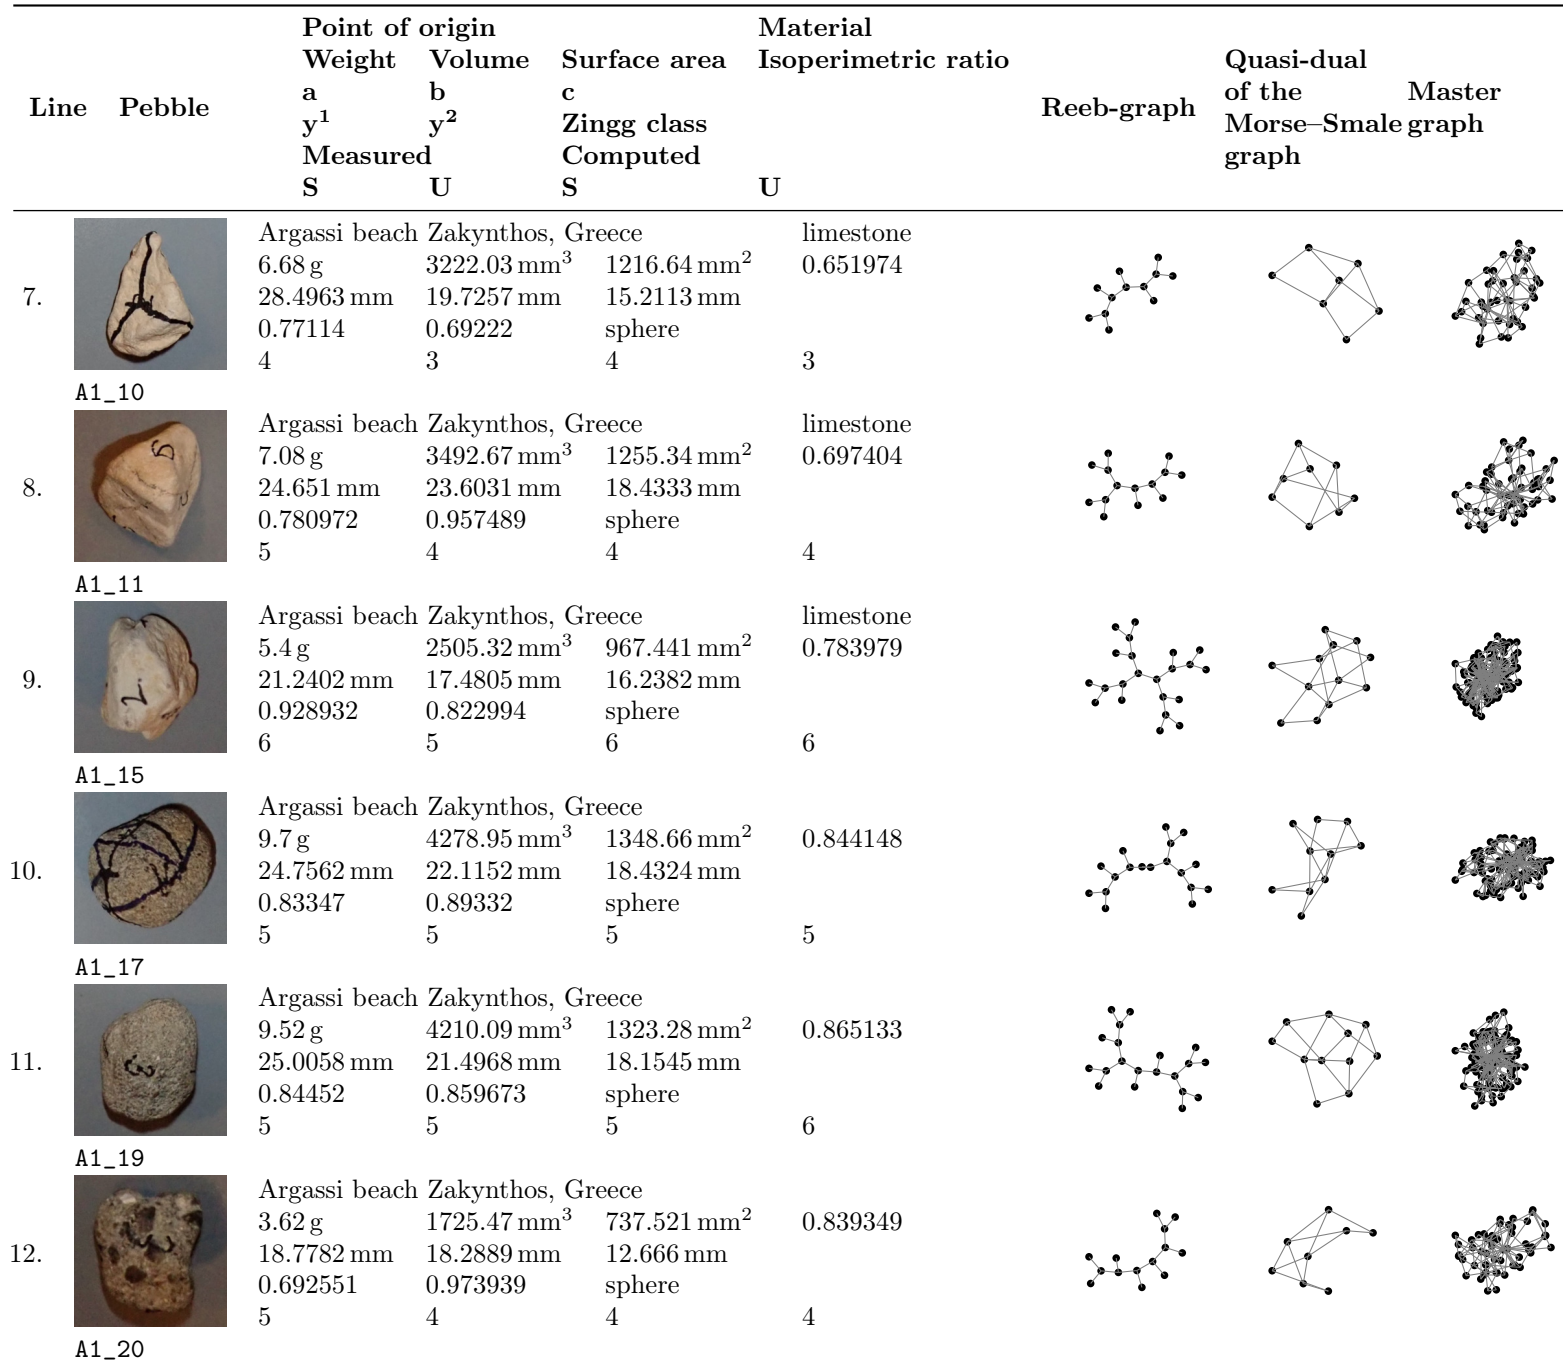   | Argassi beach<br>7.08 g<br>24.651 mm<br>0.780972<br>5  | Zakynthos, Greece<br>3492.67 mm <sup>3</sup><br>23.6031 mm<br>0.957489<br>4 | 1255.34 mm <sup>2</sup><br>18.4333 mm<br>sphere<br>4 | limestone<br>0.697404 | 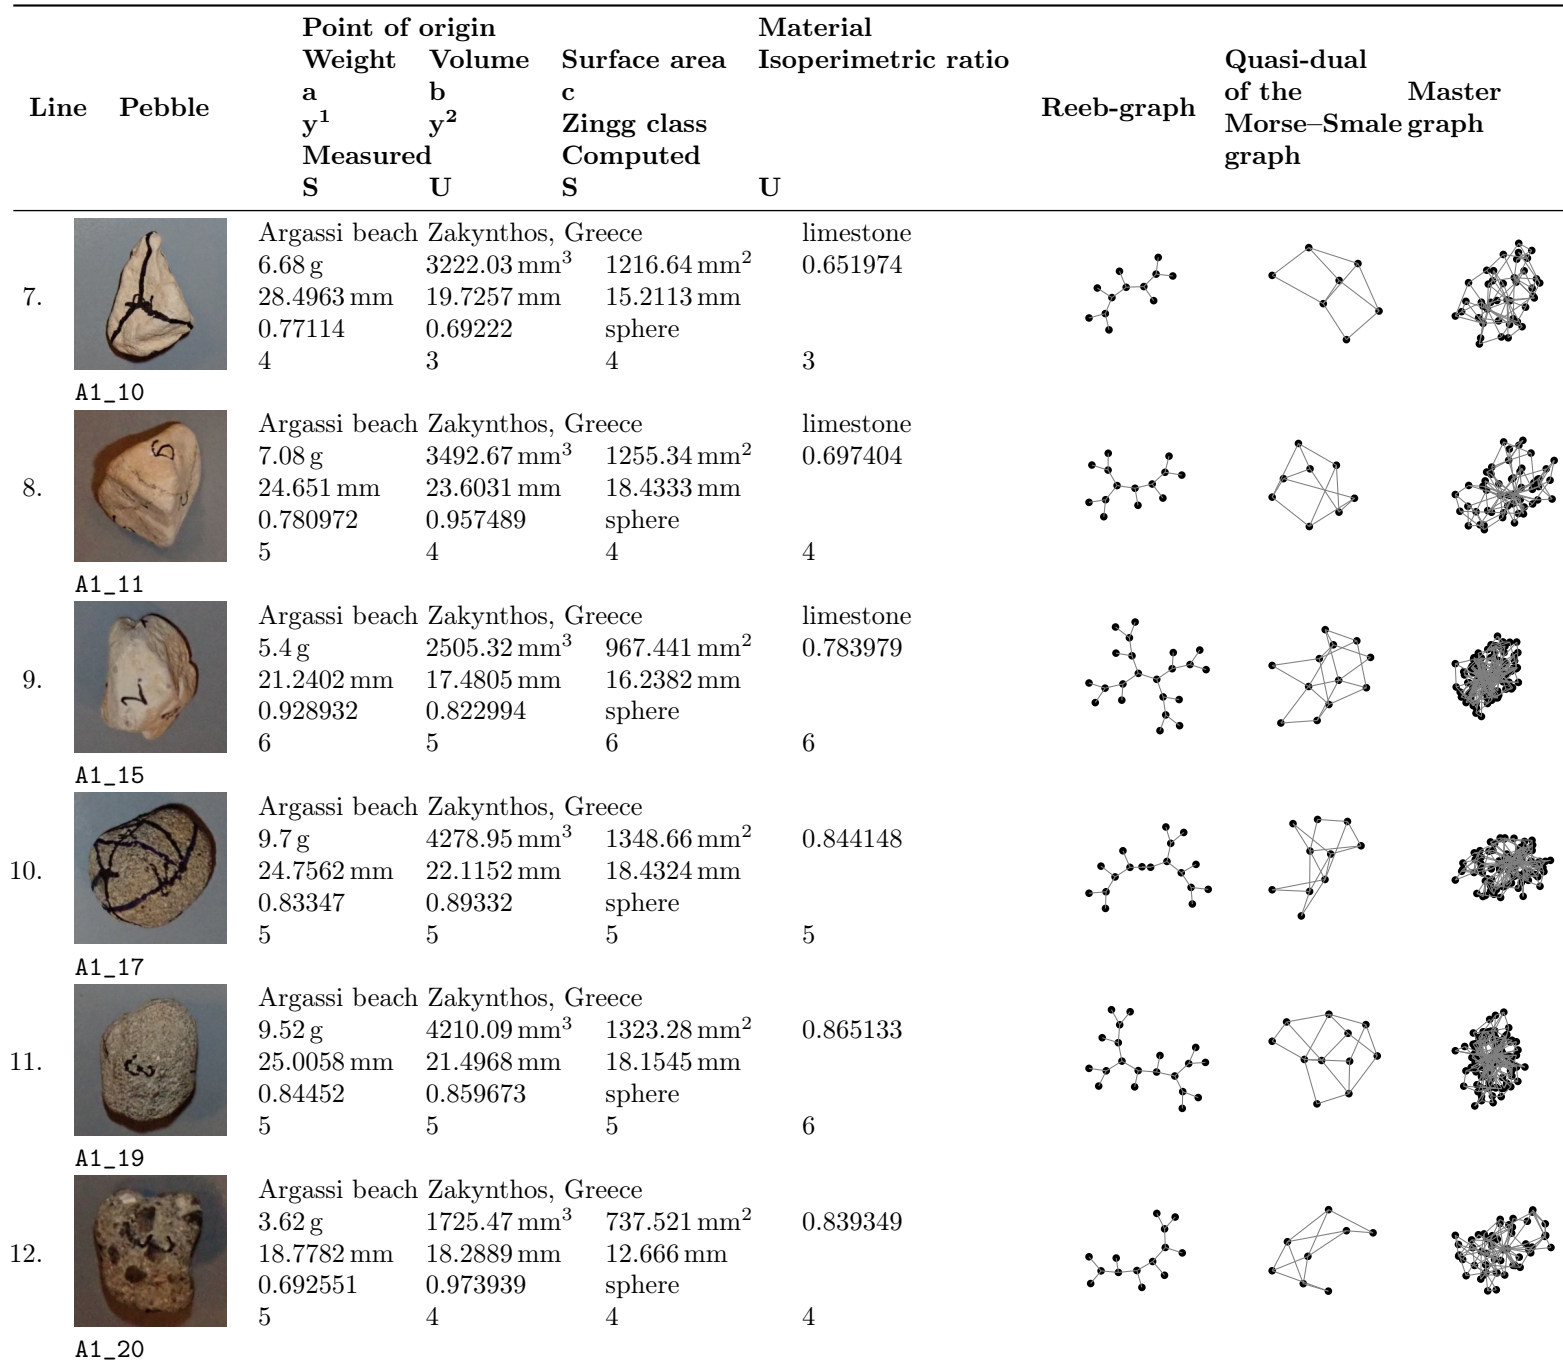   | 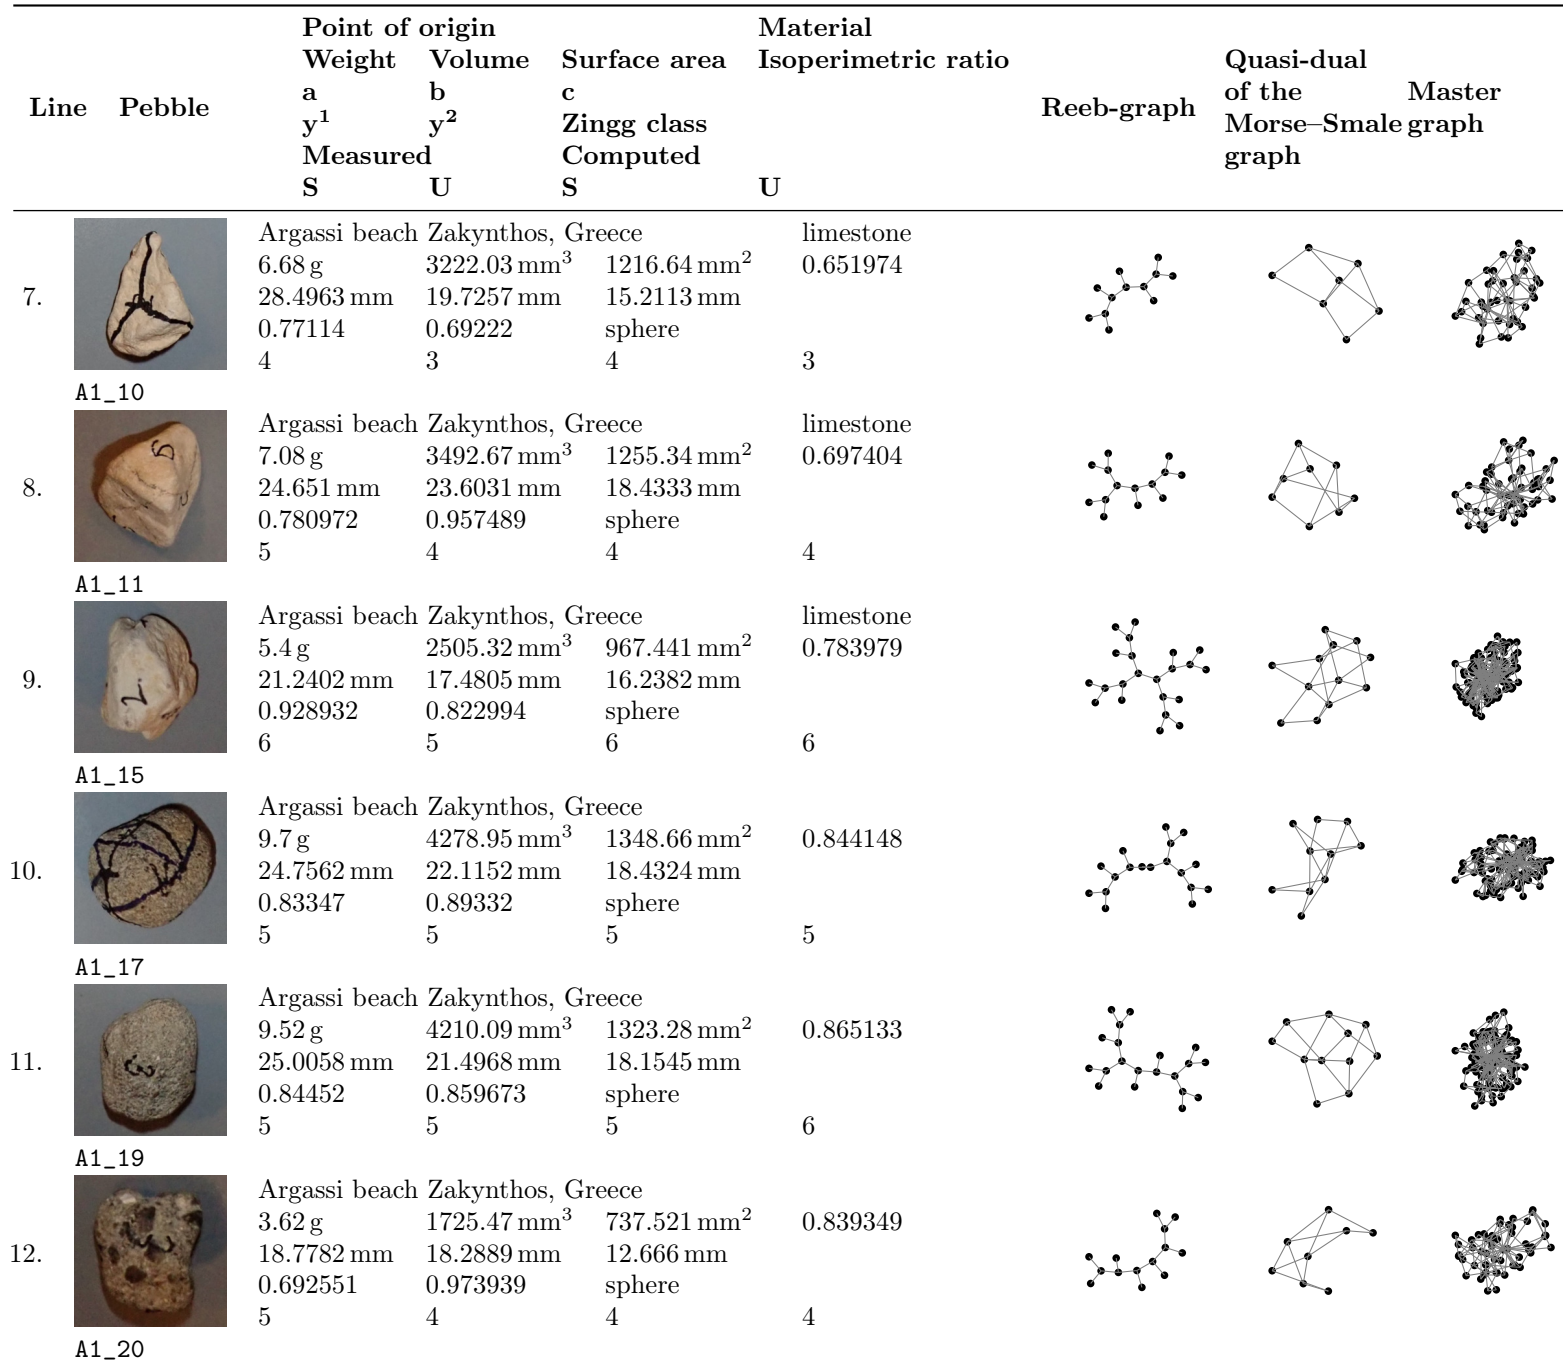   | 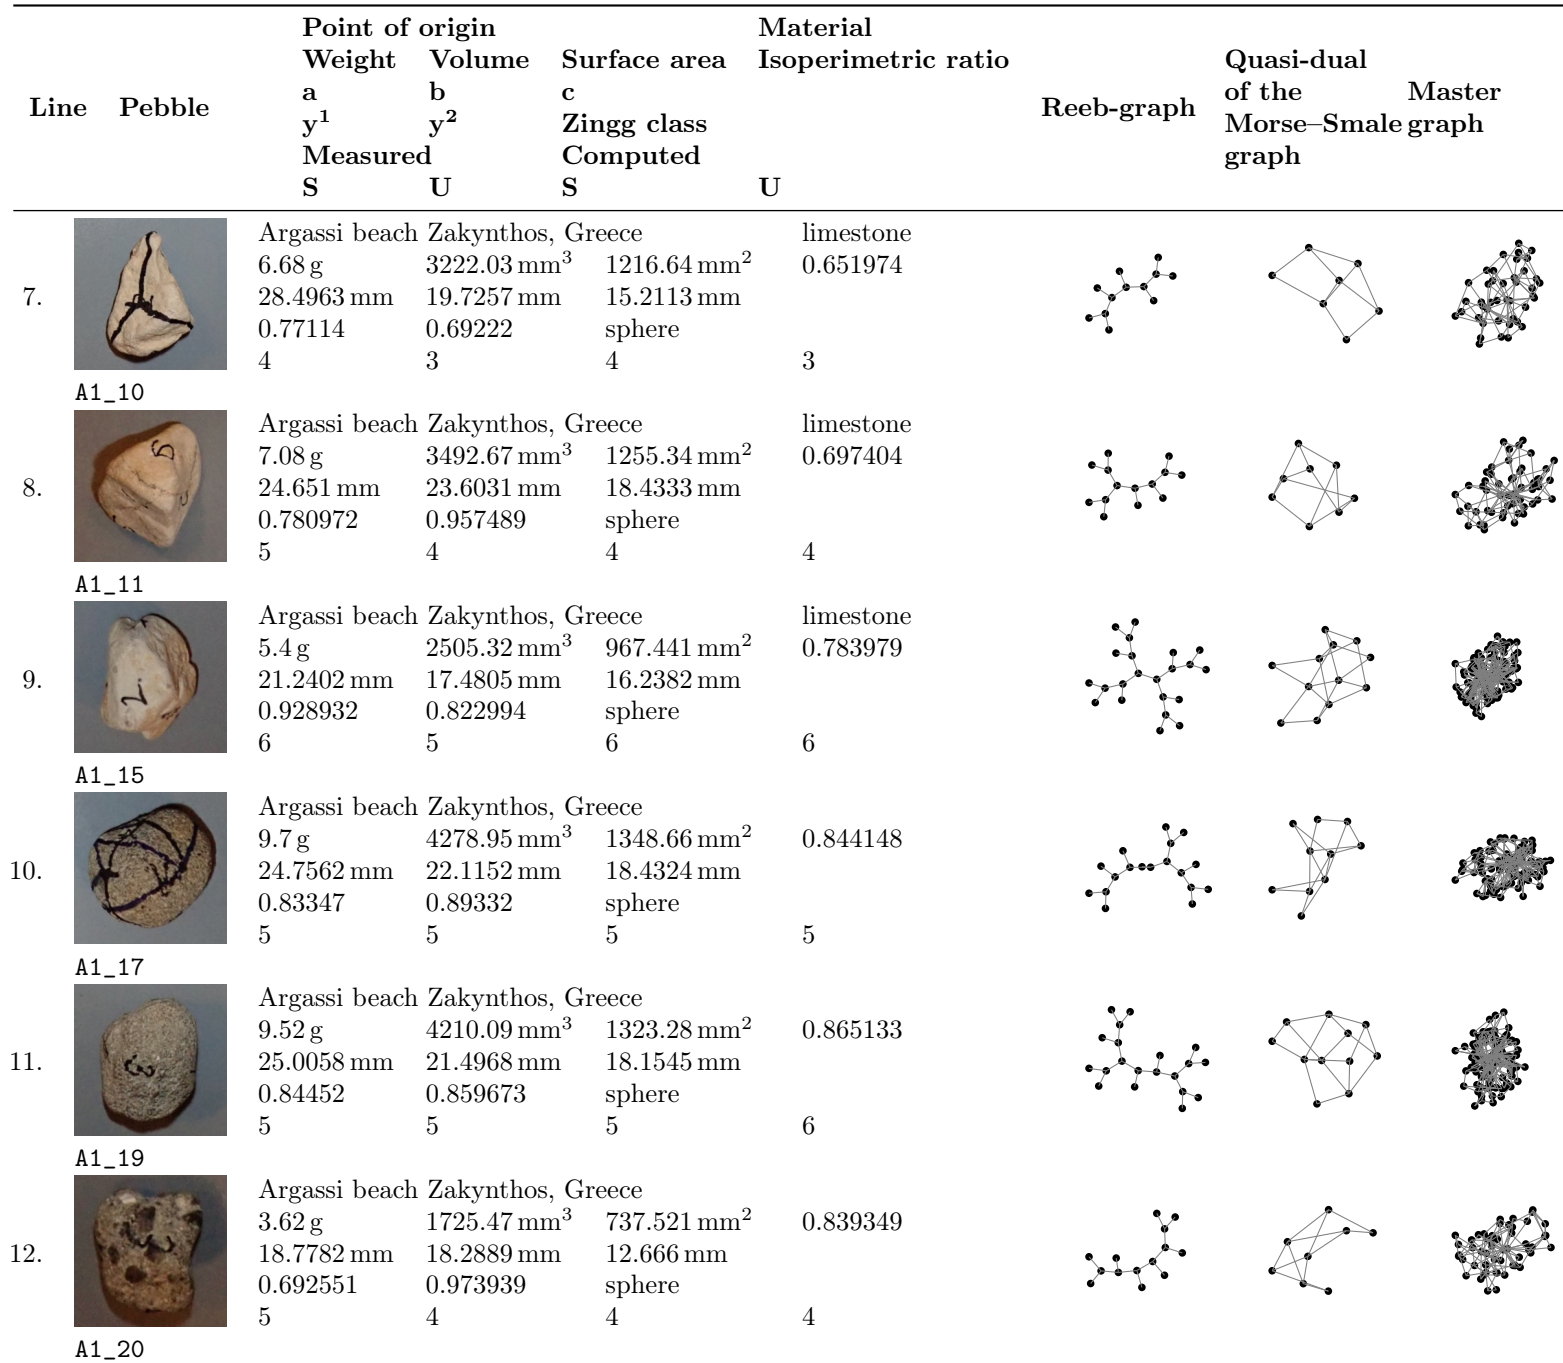   |
| A1_11 |                                                                                     |                                                        |                                                                             |                                                      |                       |                                                                                       |                                                                                       |                                                                                       |
| 9.    | 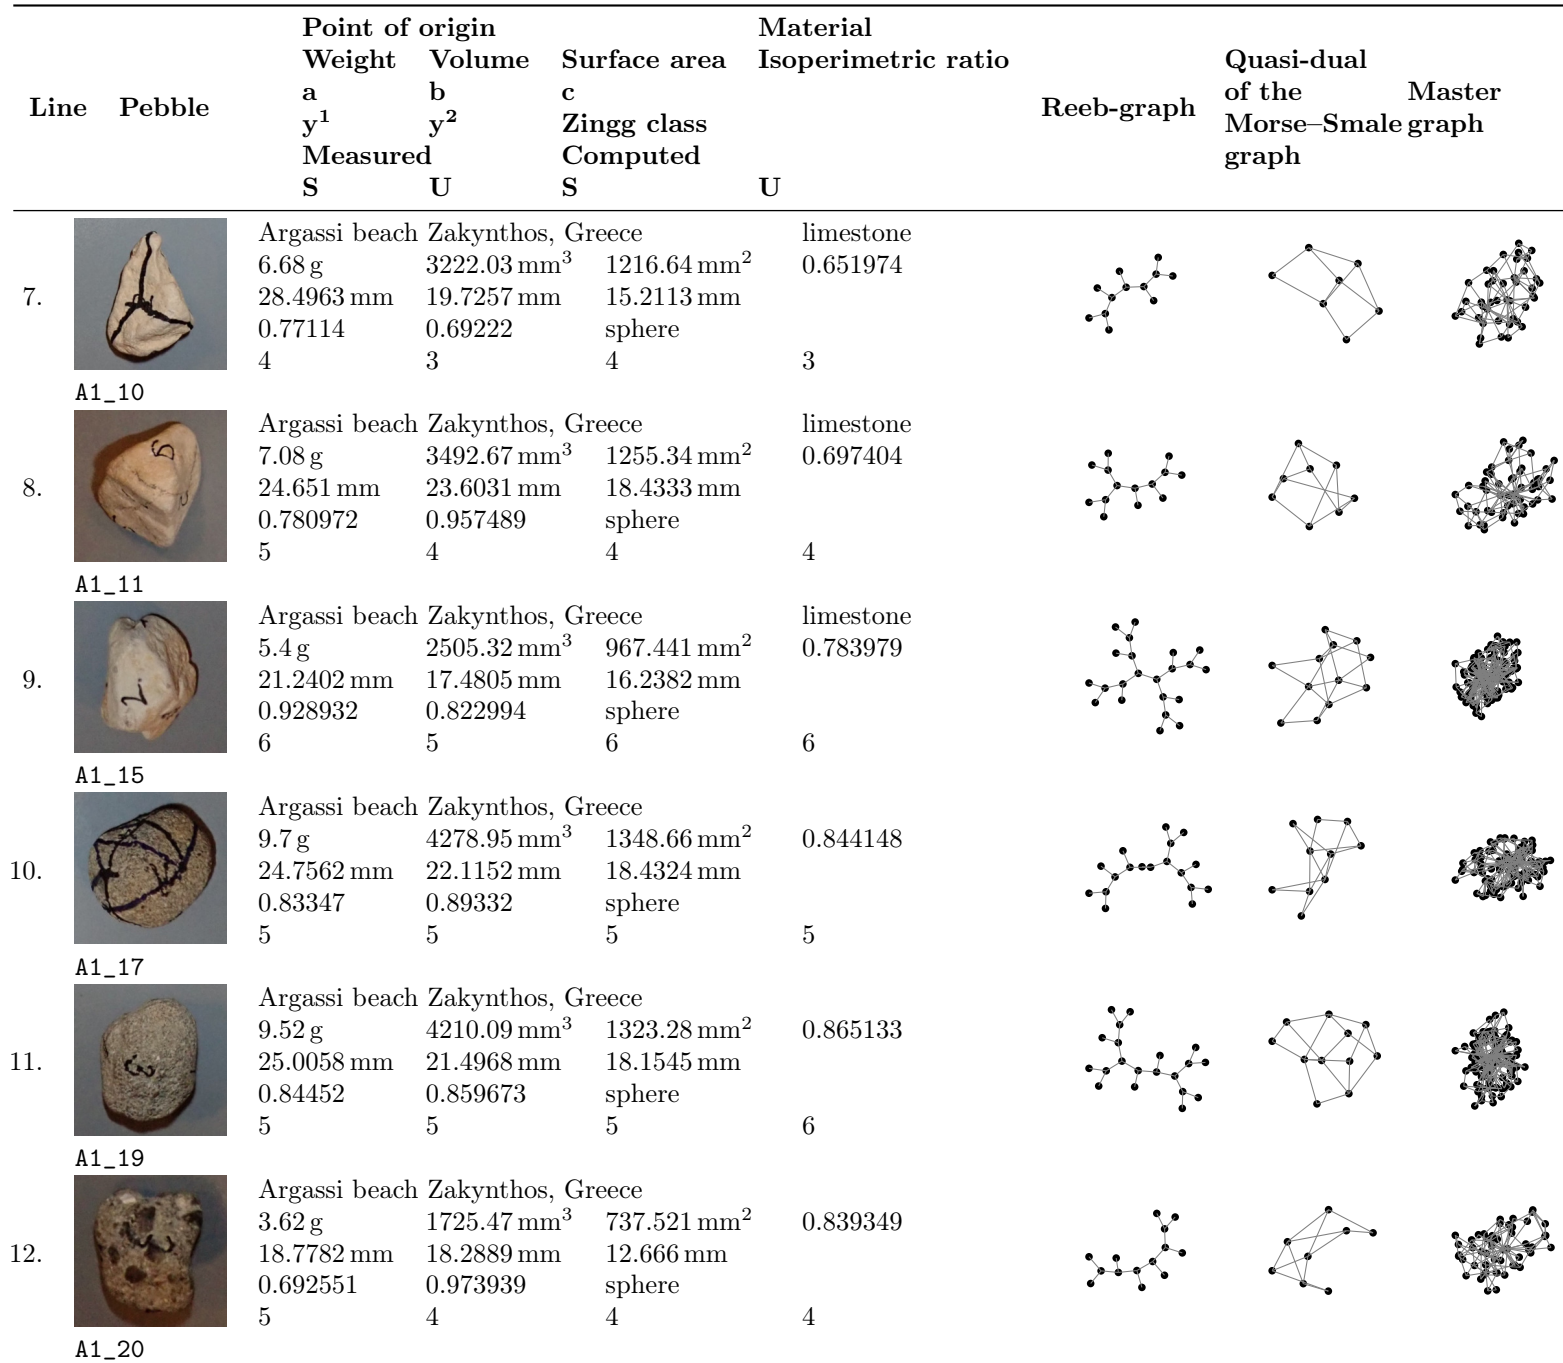   | Argassi beach<br>5.4 g<br>21.2402 mm<br>0.928932<br>6  | Zakynthos, Greece<br>2505.32 mm <sup>3</sup><br>17.4805 mm<br>0.822994<br>5 | 967.441 mm <sup>2</sup><br>16.2382 mm<br>sphere<br>6 | limestone<br>0.783979 | 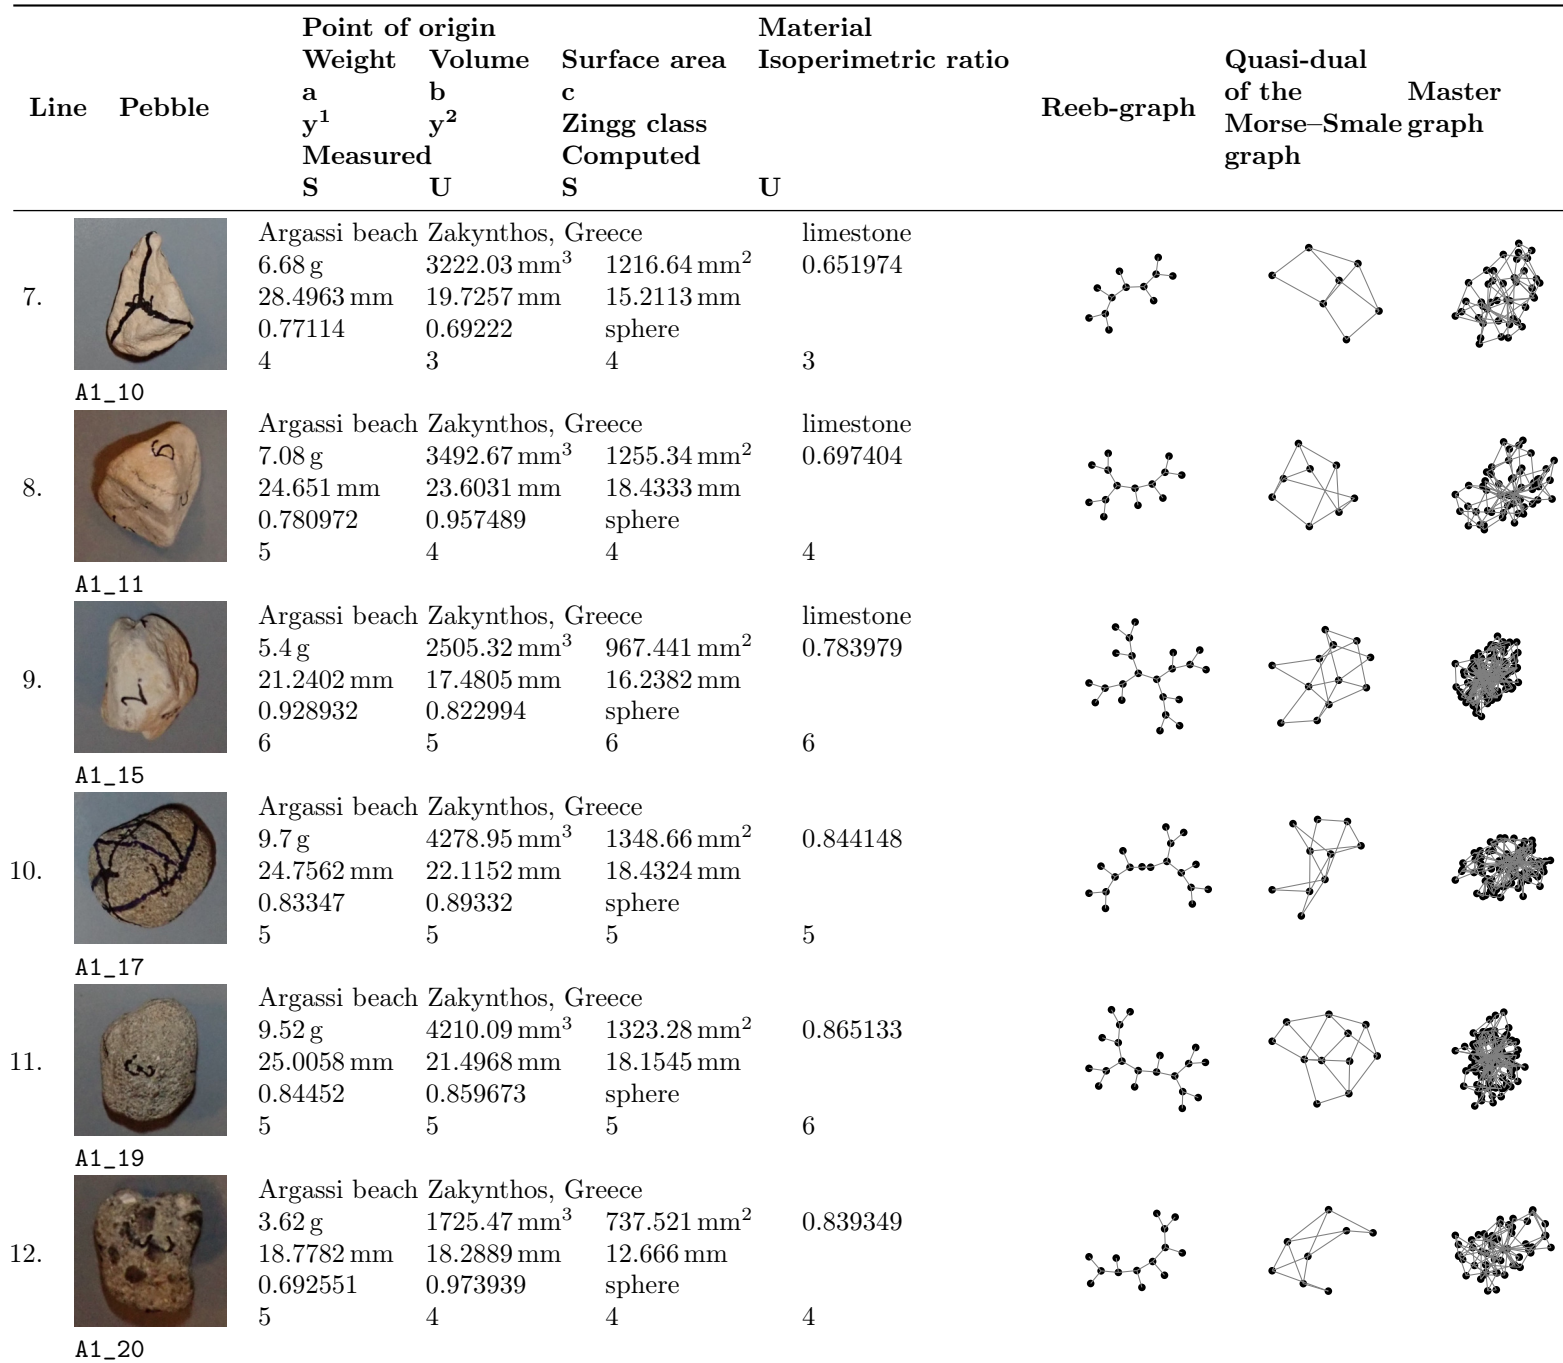   | 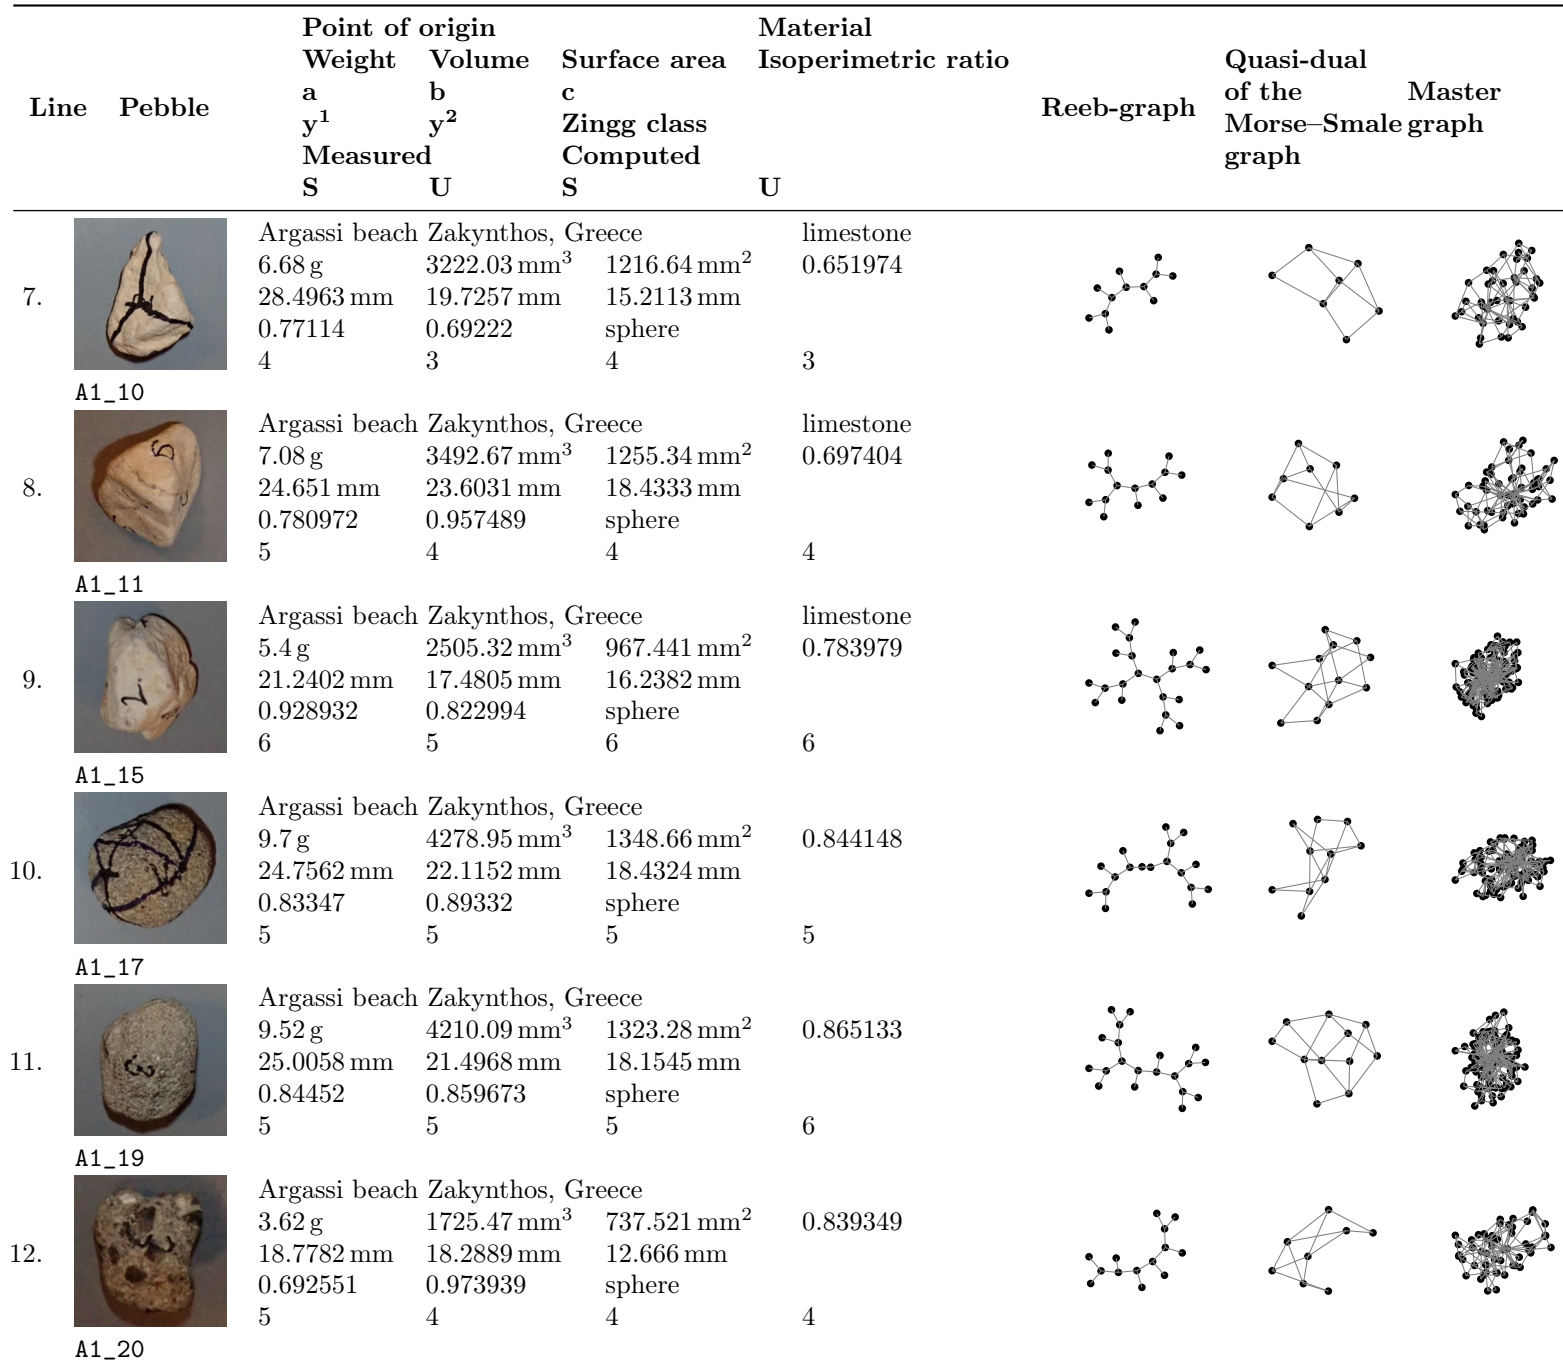   | 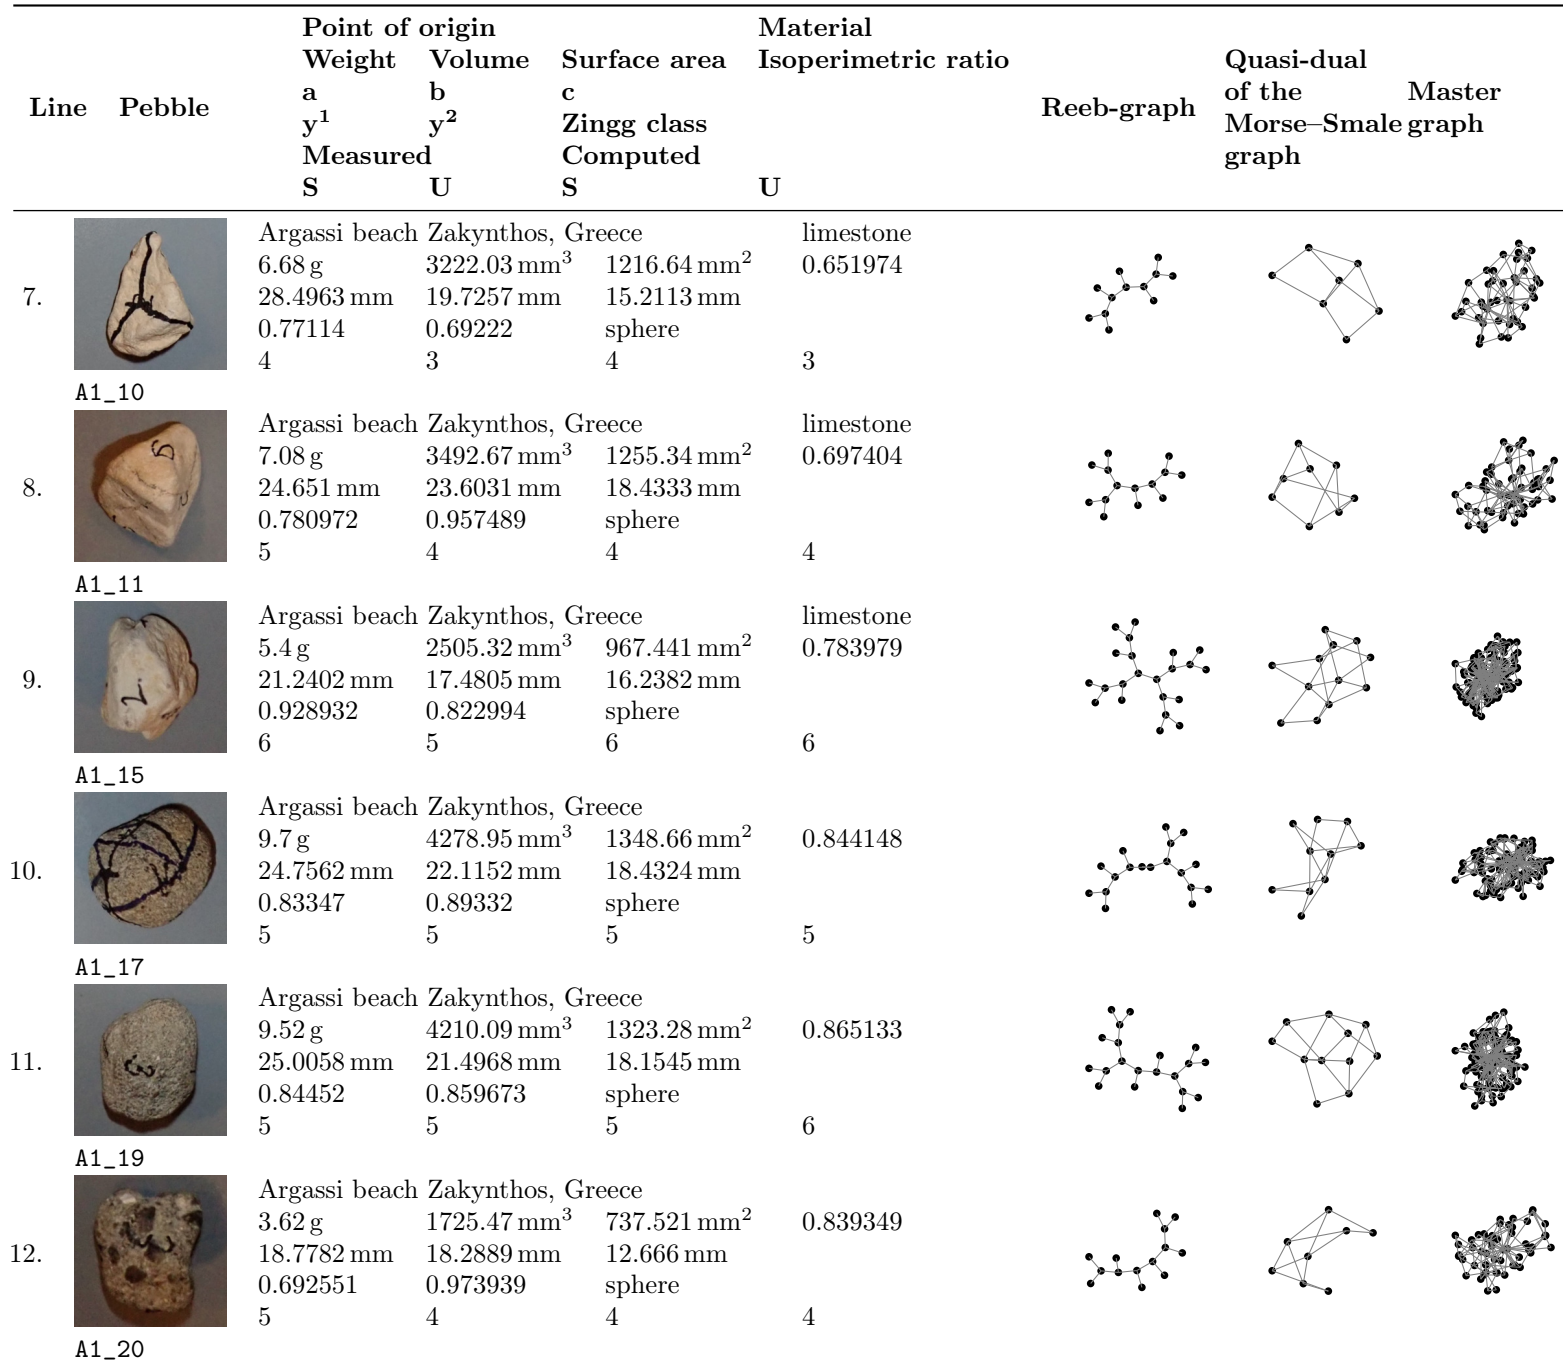   |
| A1_15 |                                                                                     |                                                        |                                                                             |                                                      |                       |                                                                                       |                                                                                       |                                                                                       |
| 10.   | 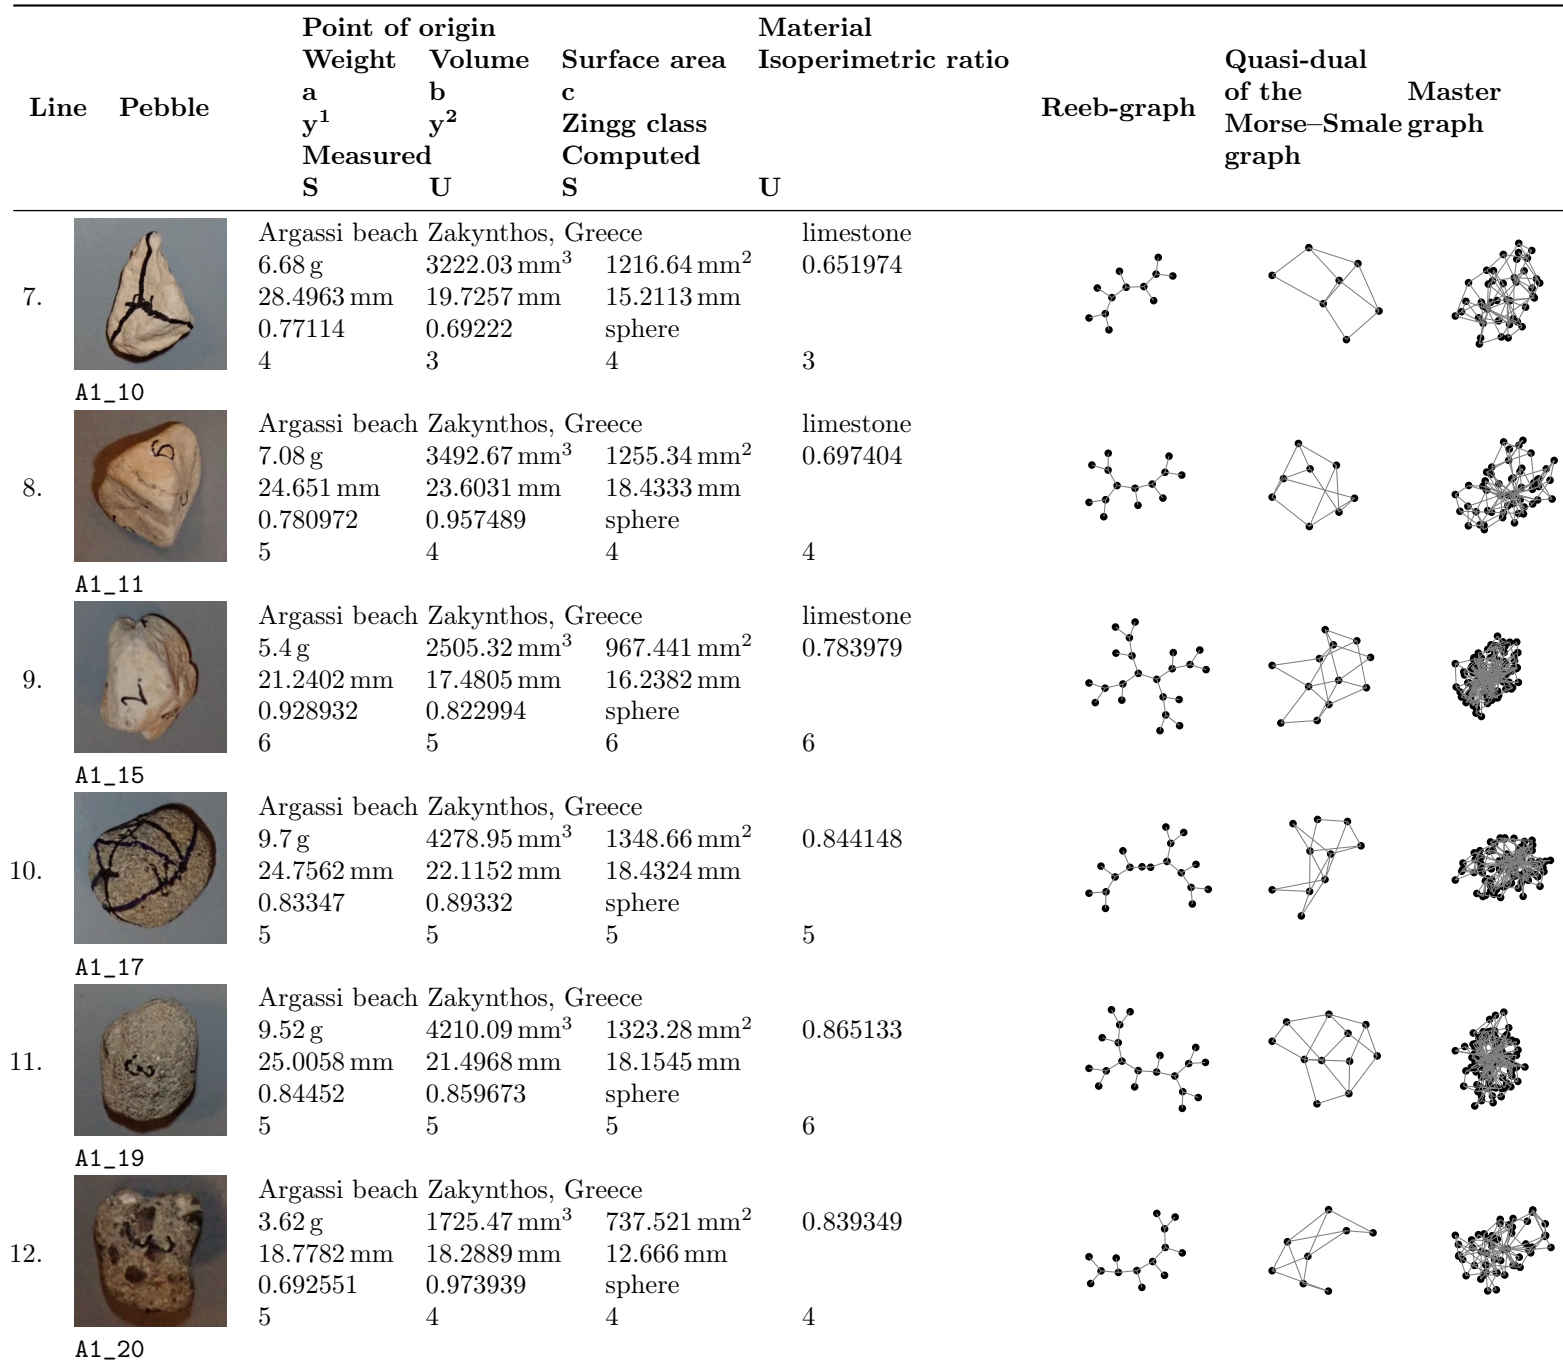  | Argassi beach<br>9.7 g<br>24.7562 mm<br>0.83347<br>5   | Zakynthos, Greece<br>4278.95 mm <sup>3</sup><br>22.1152 mm<br>0.89332<br>5  | 1348.66 mm <sup>2</sup><br>18.4324 mm<br>sphere<br>5 | 0.844148              | 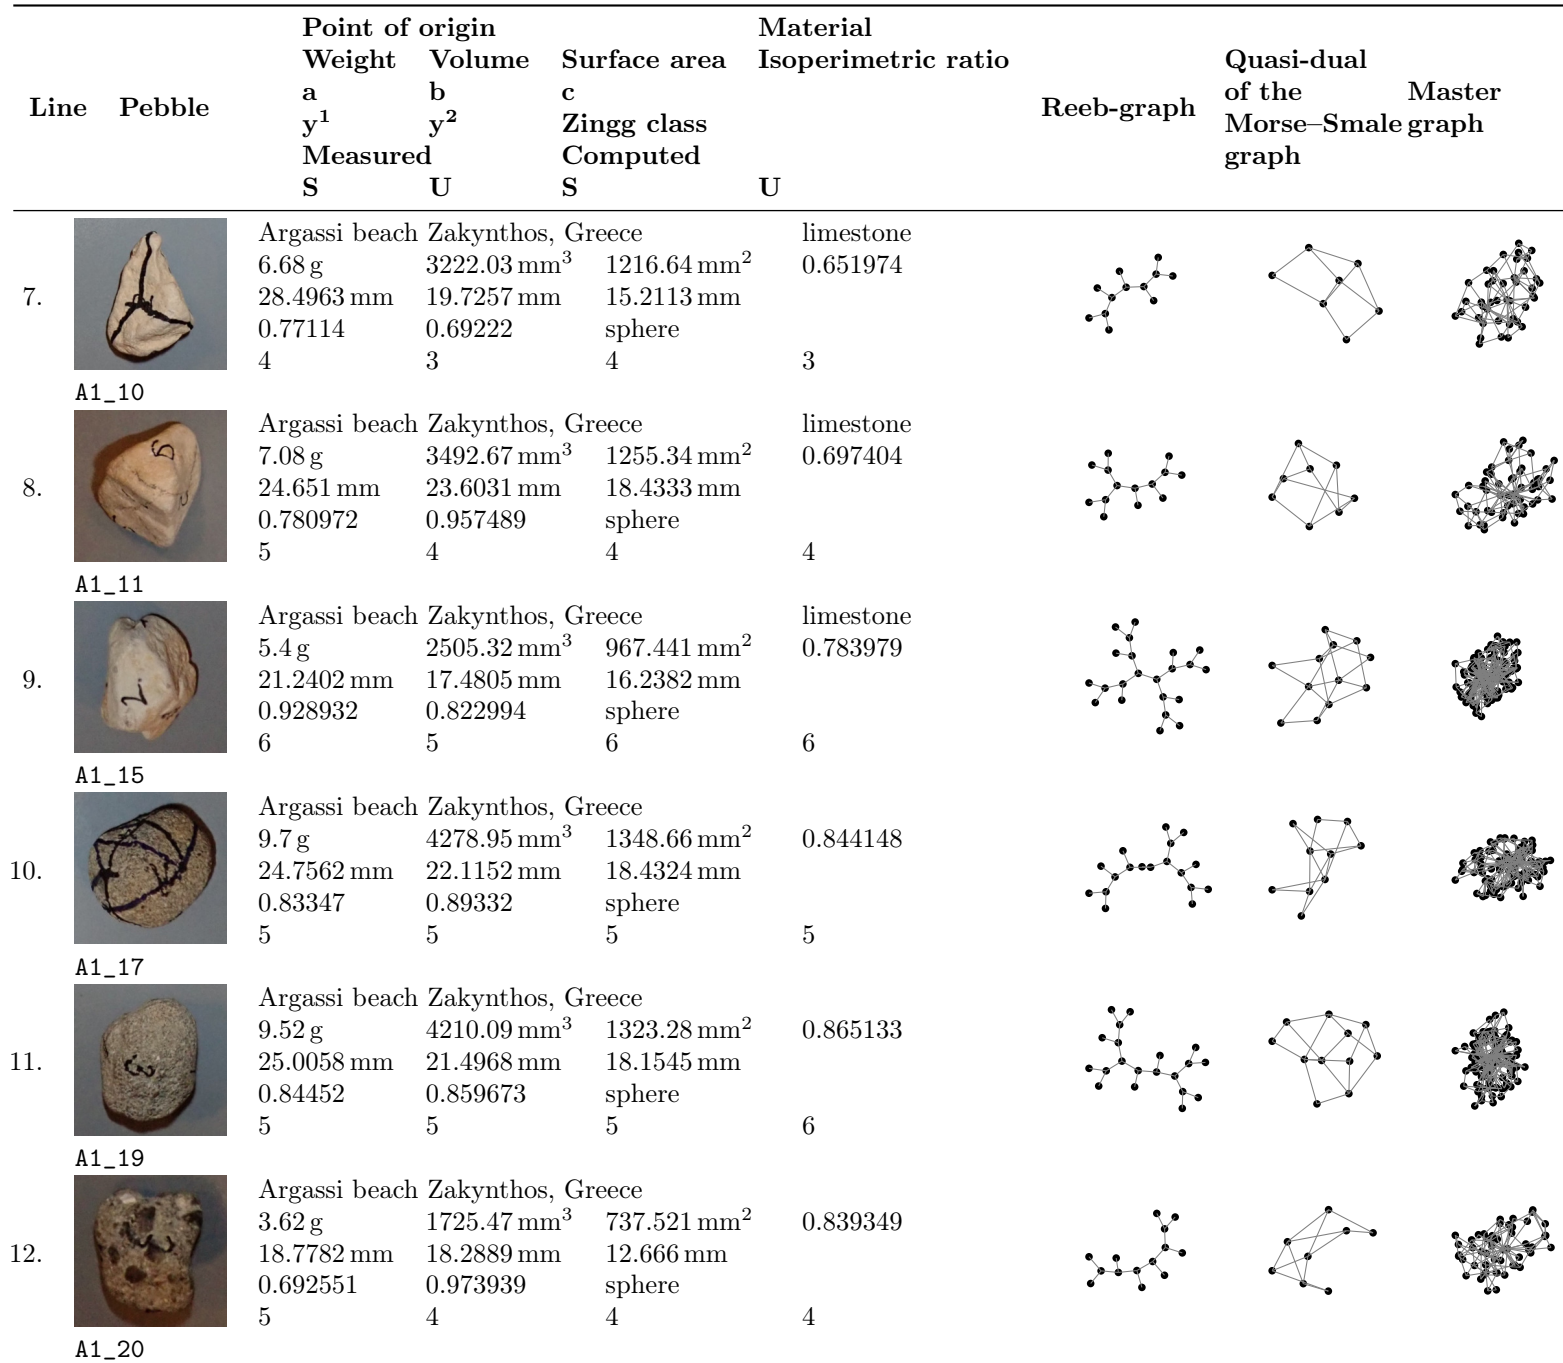  | 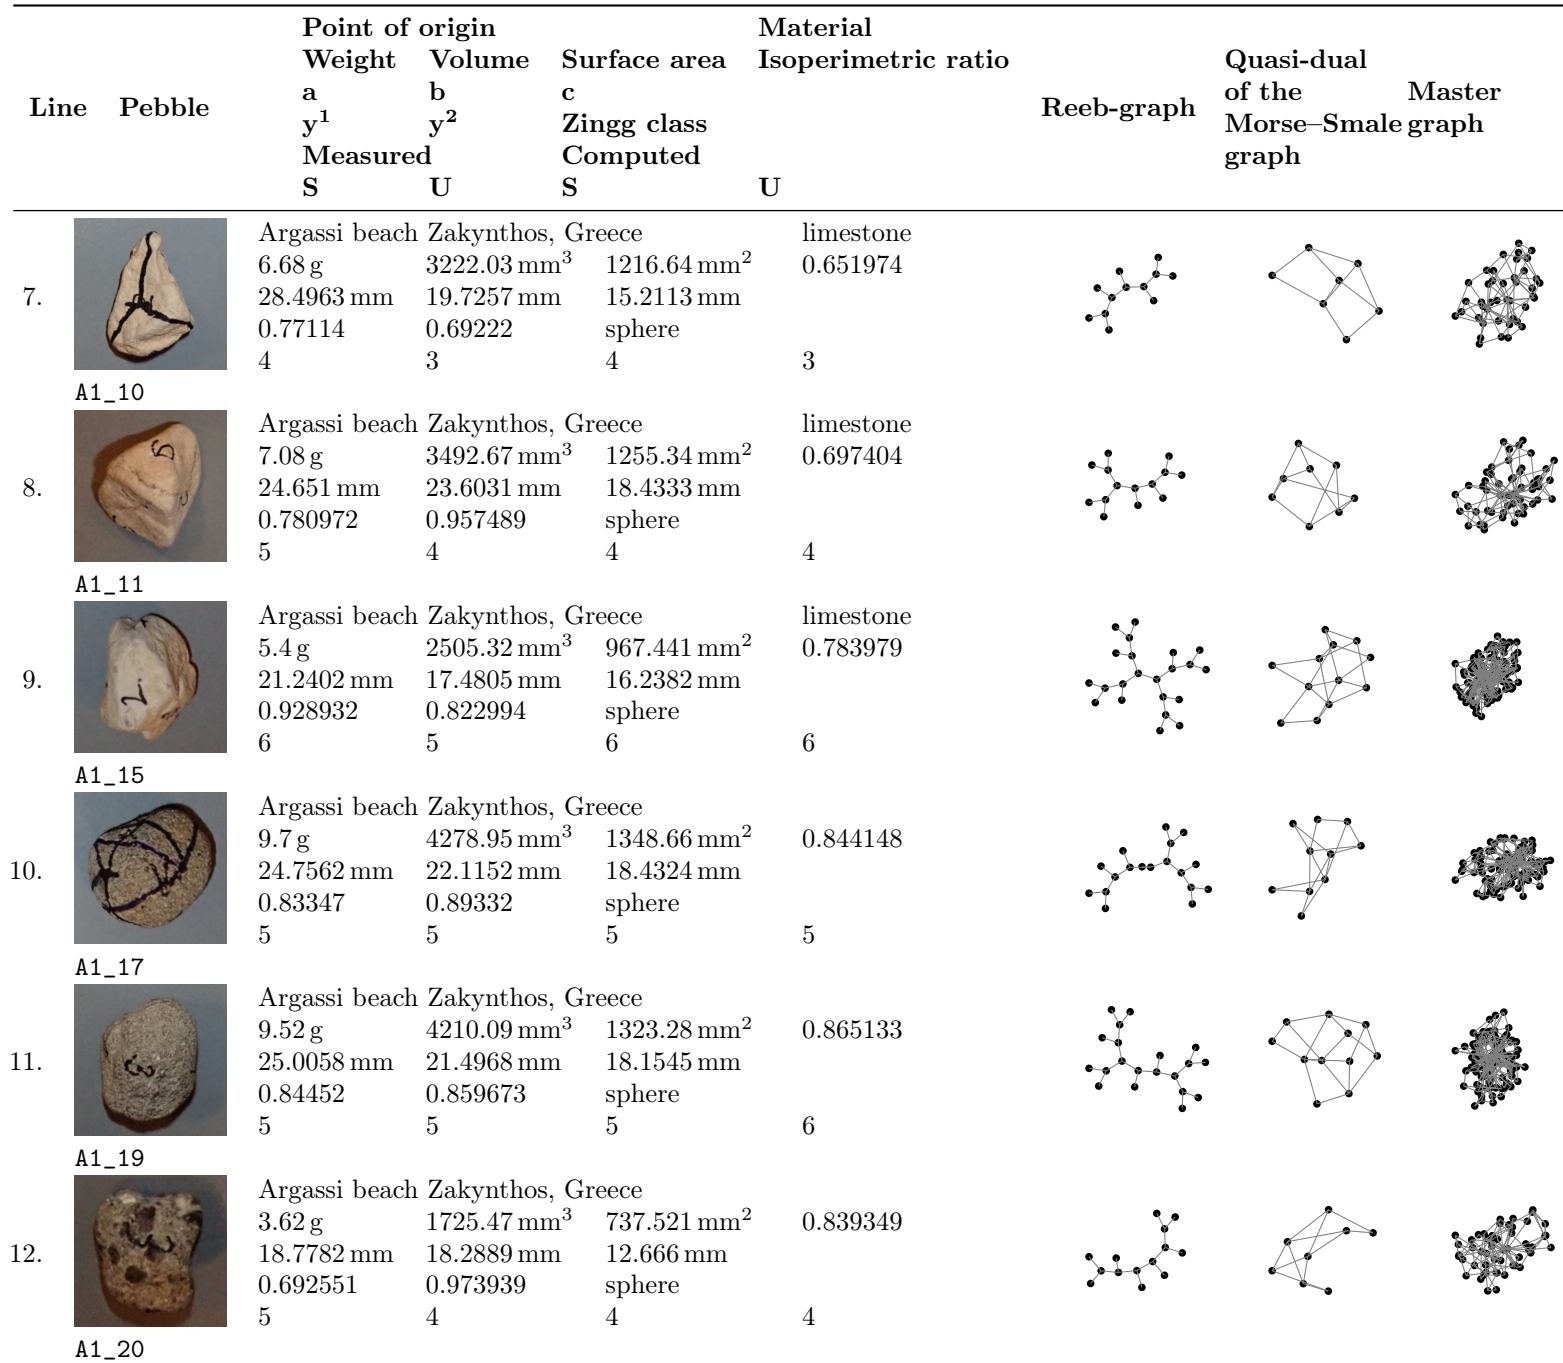  | 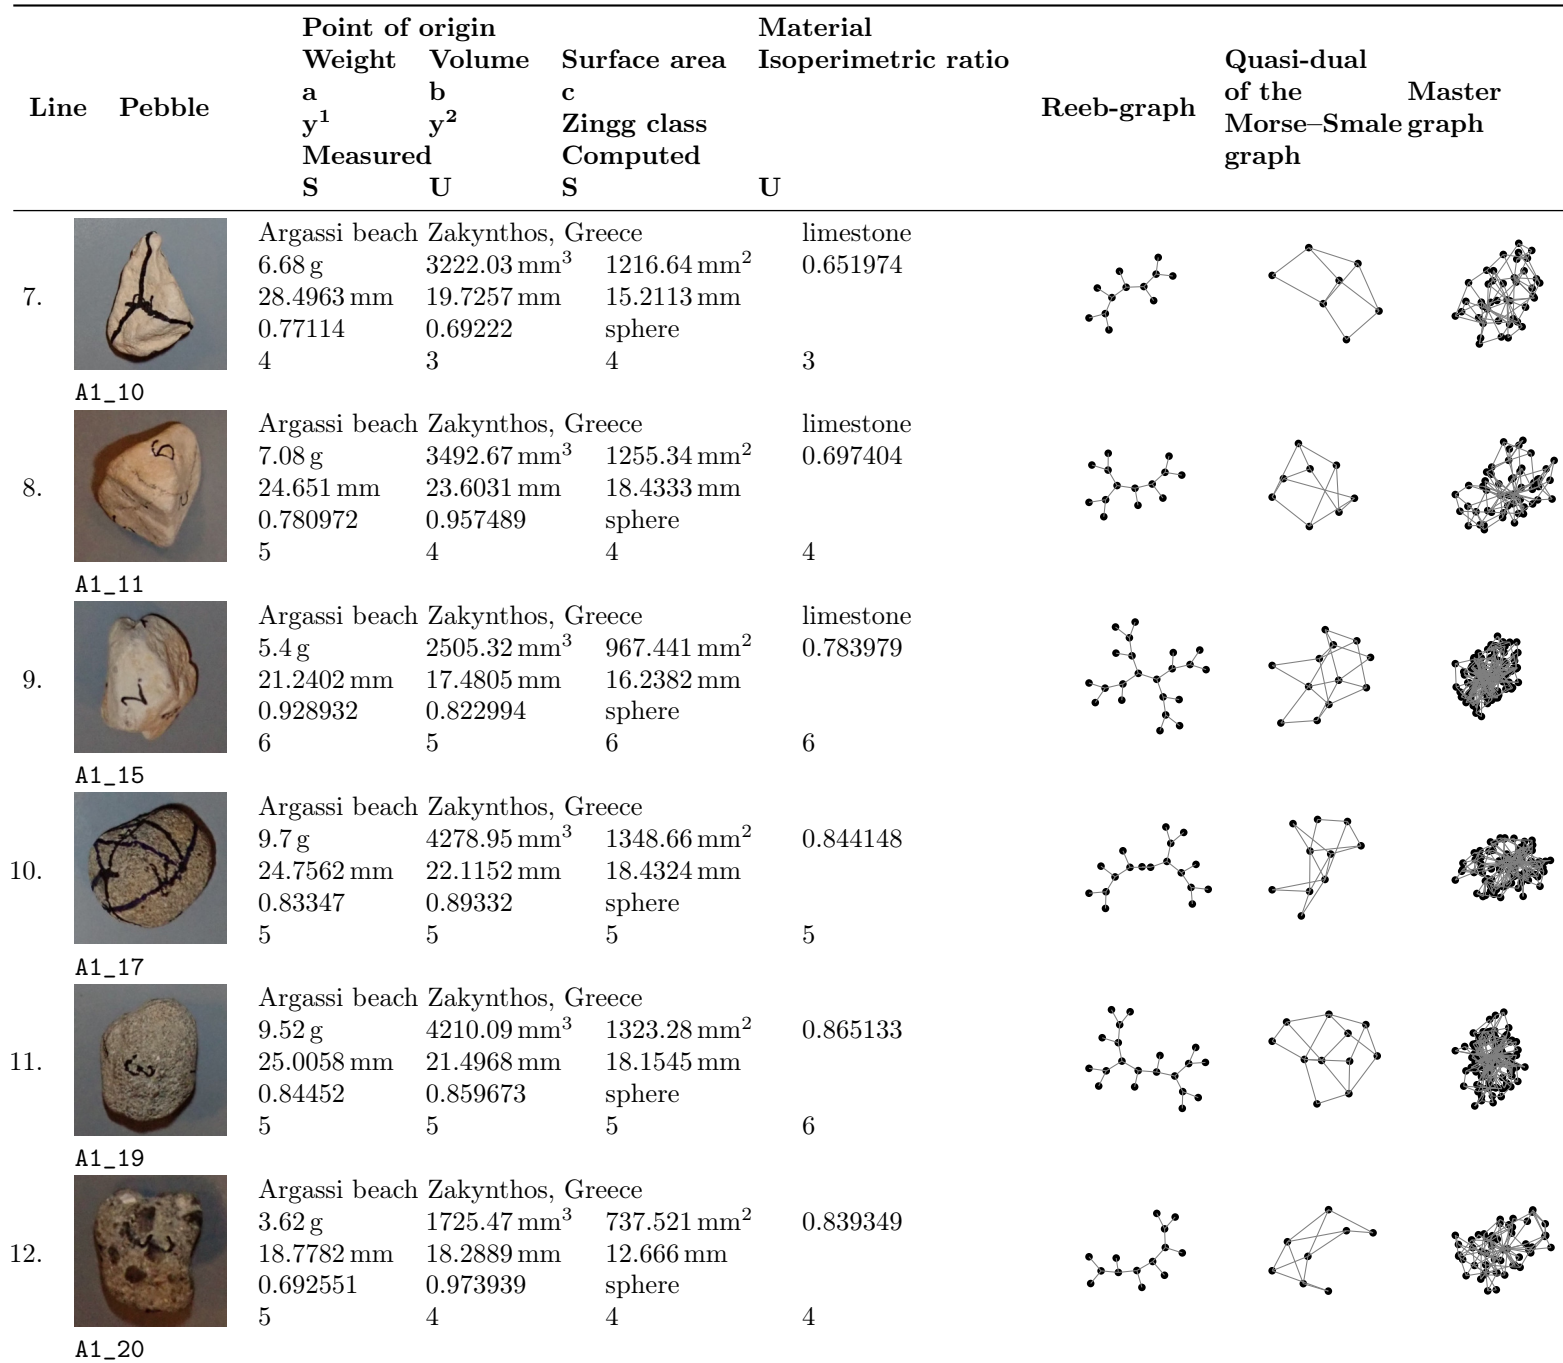  |
| A1_17 |                                                                                     |                                                        |                                                                             |                                                      |                       |                                                                                       |                                                                                       |                                                                                       |
| 11.   | 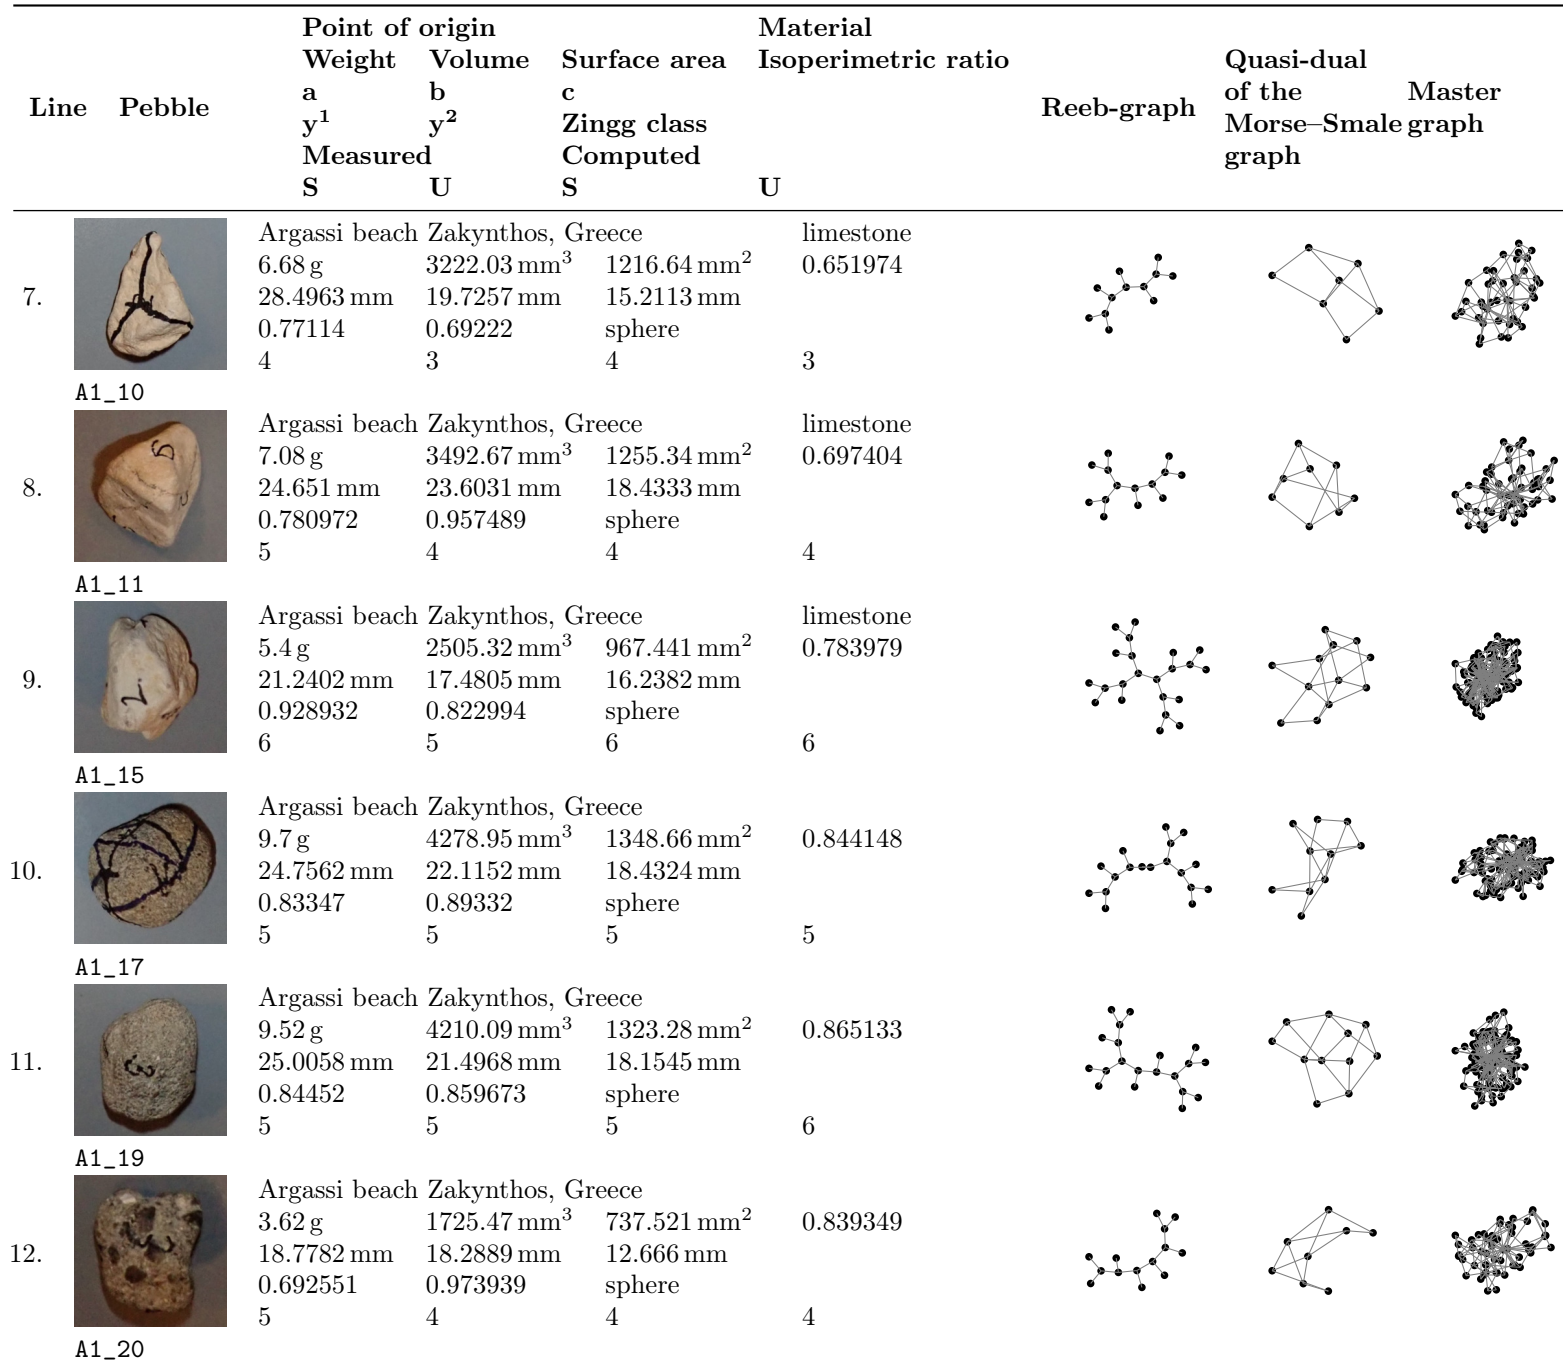 | Argassi beach<br>9.52 g<br>25.0058 mm<br>0.84452<br>5  | Zakynthos, Greece<br>4210.09 mm <sup>3</sup><br>21.4968 mm<br>0.859673<br>5 | 1323.28 mm <sup>2</sup><br>18.1545 mm<br>sphere<br>5 | 0.865133              | 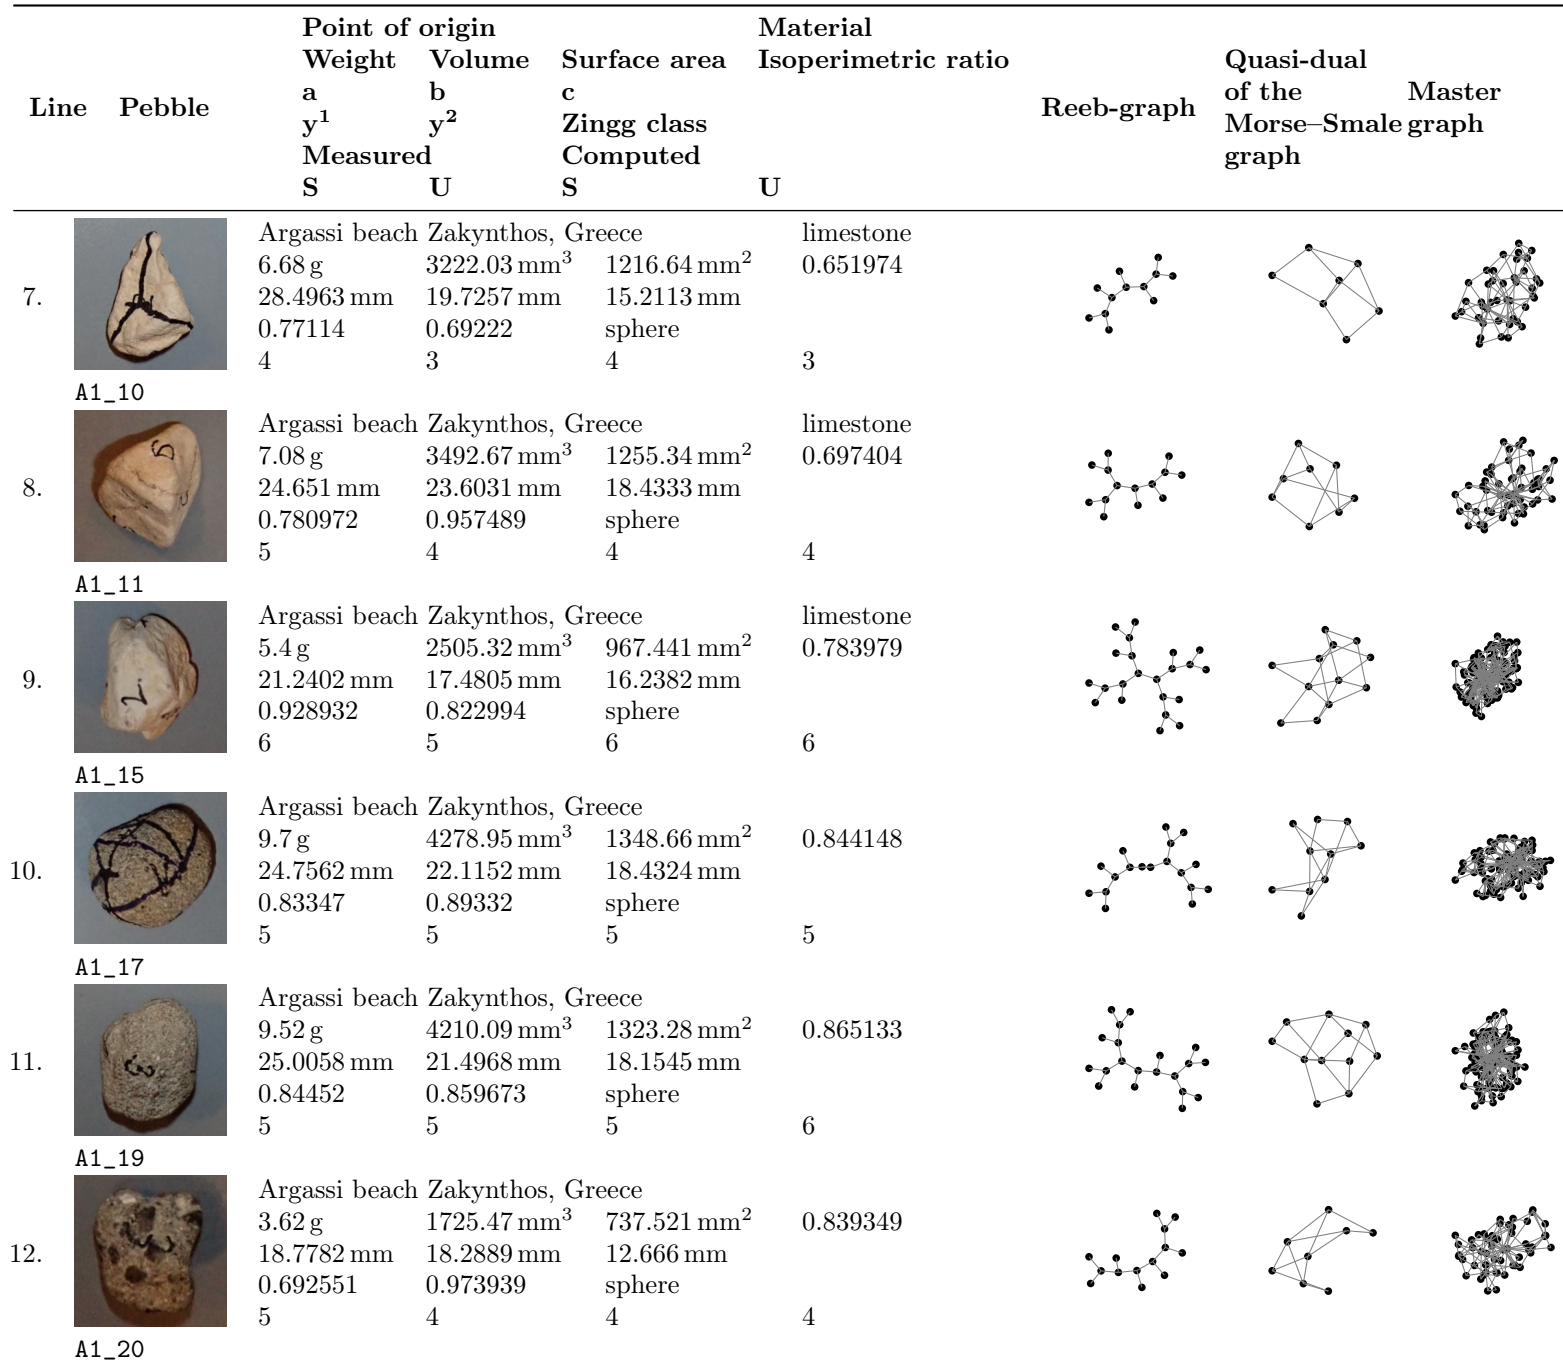 | 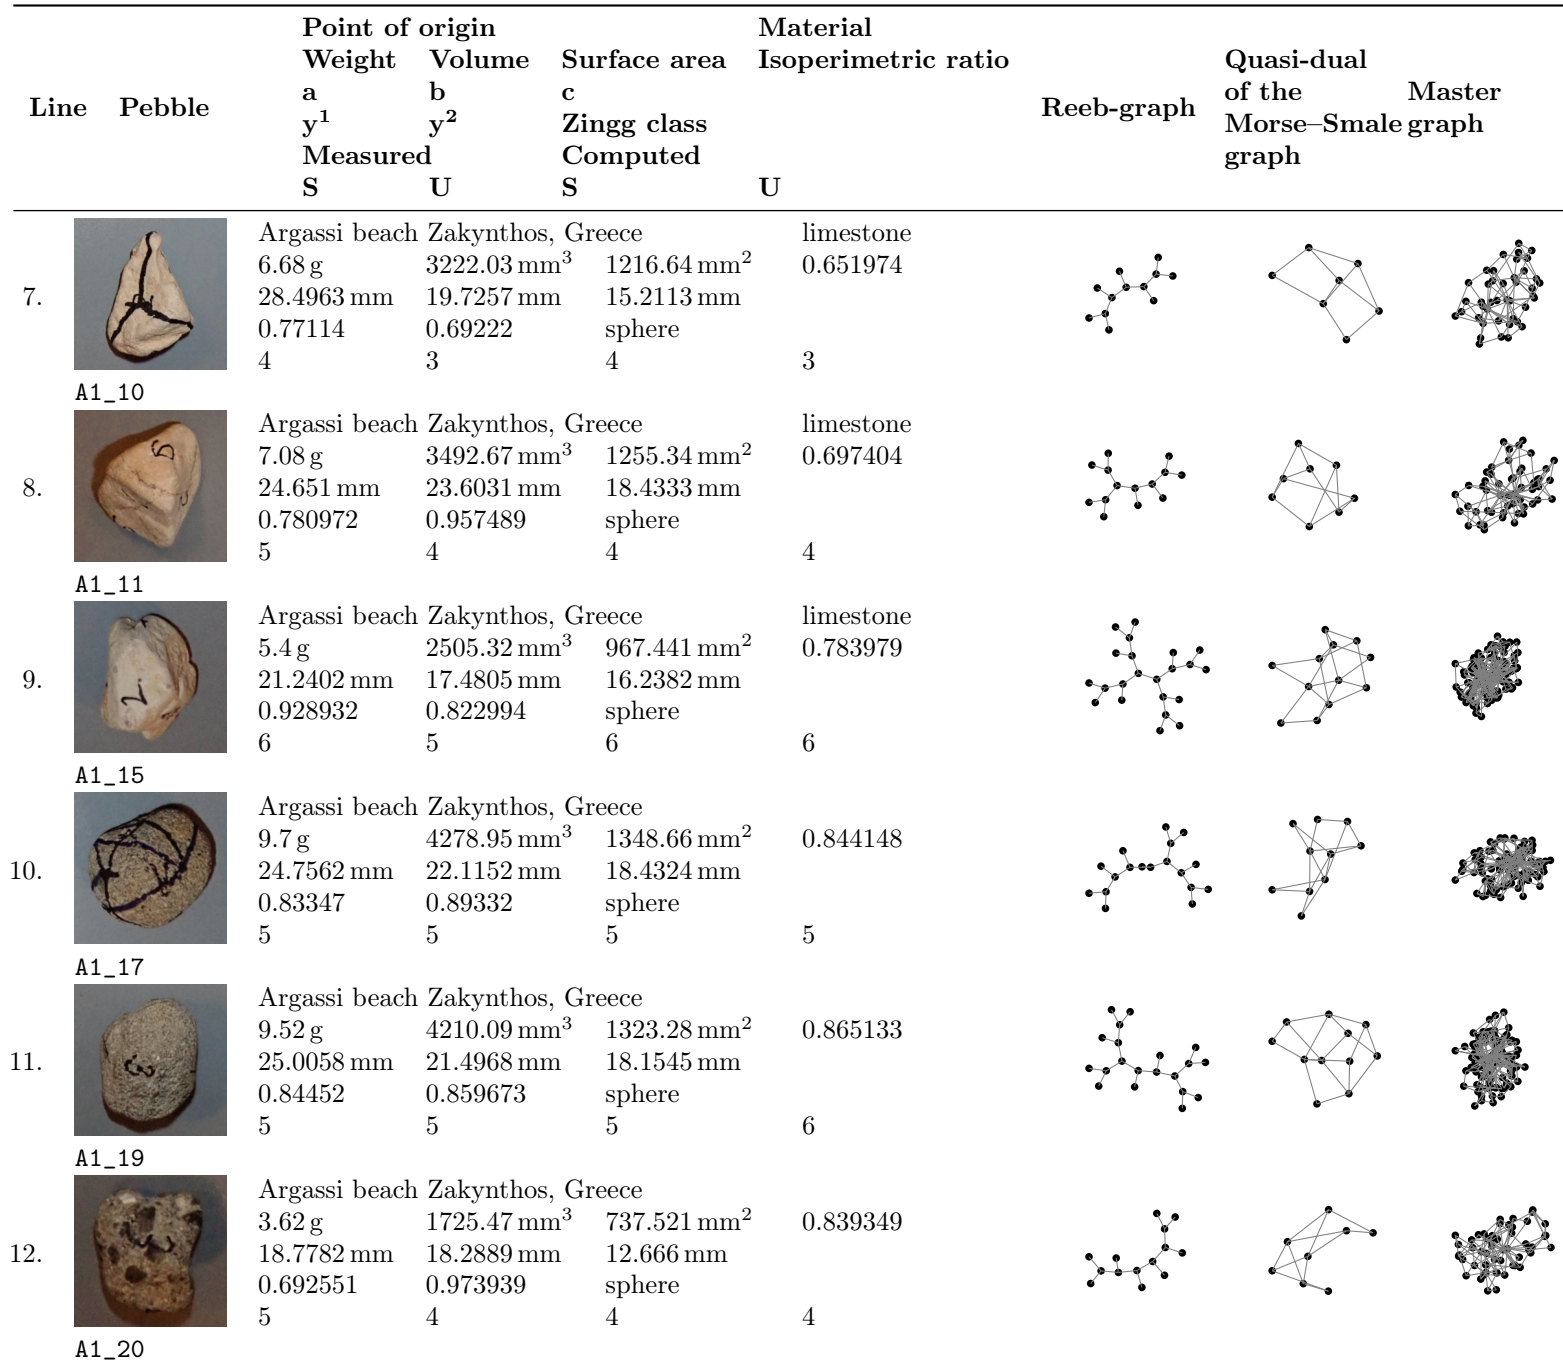 | 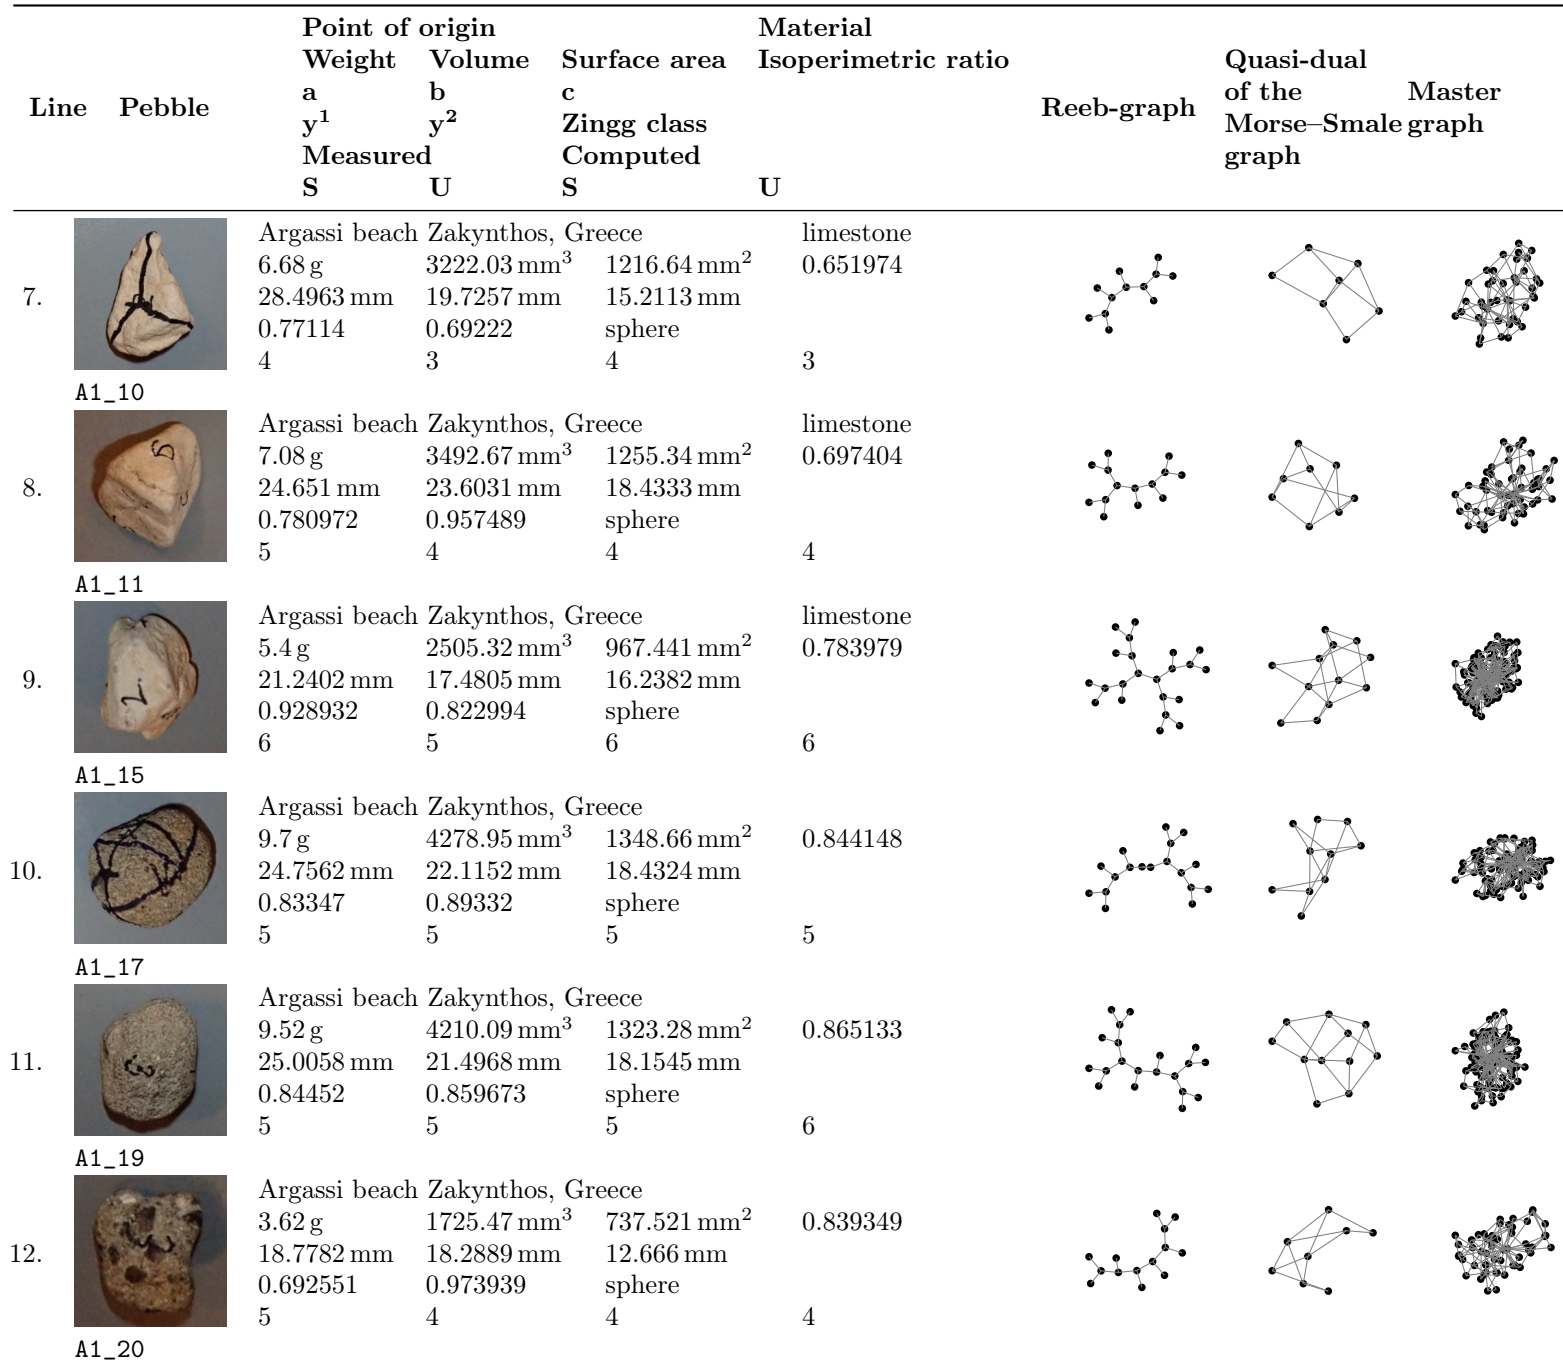 |
| A1_19 |                                                                                     |                                                        |                                                                             |                                                      |                       |                                                                                       |                                                                                       |                                                                                       |
| 12.   | 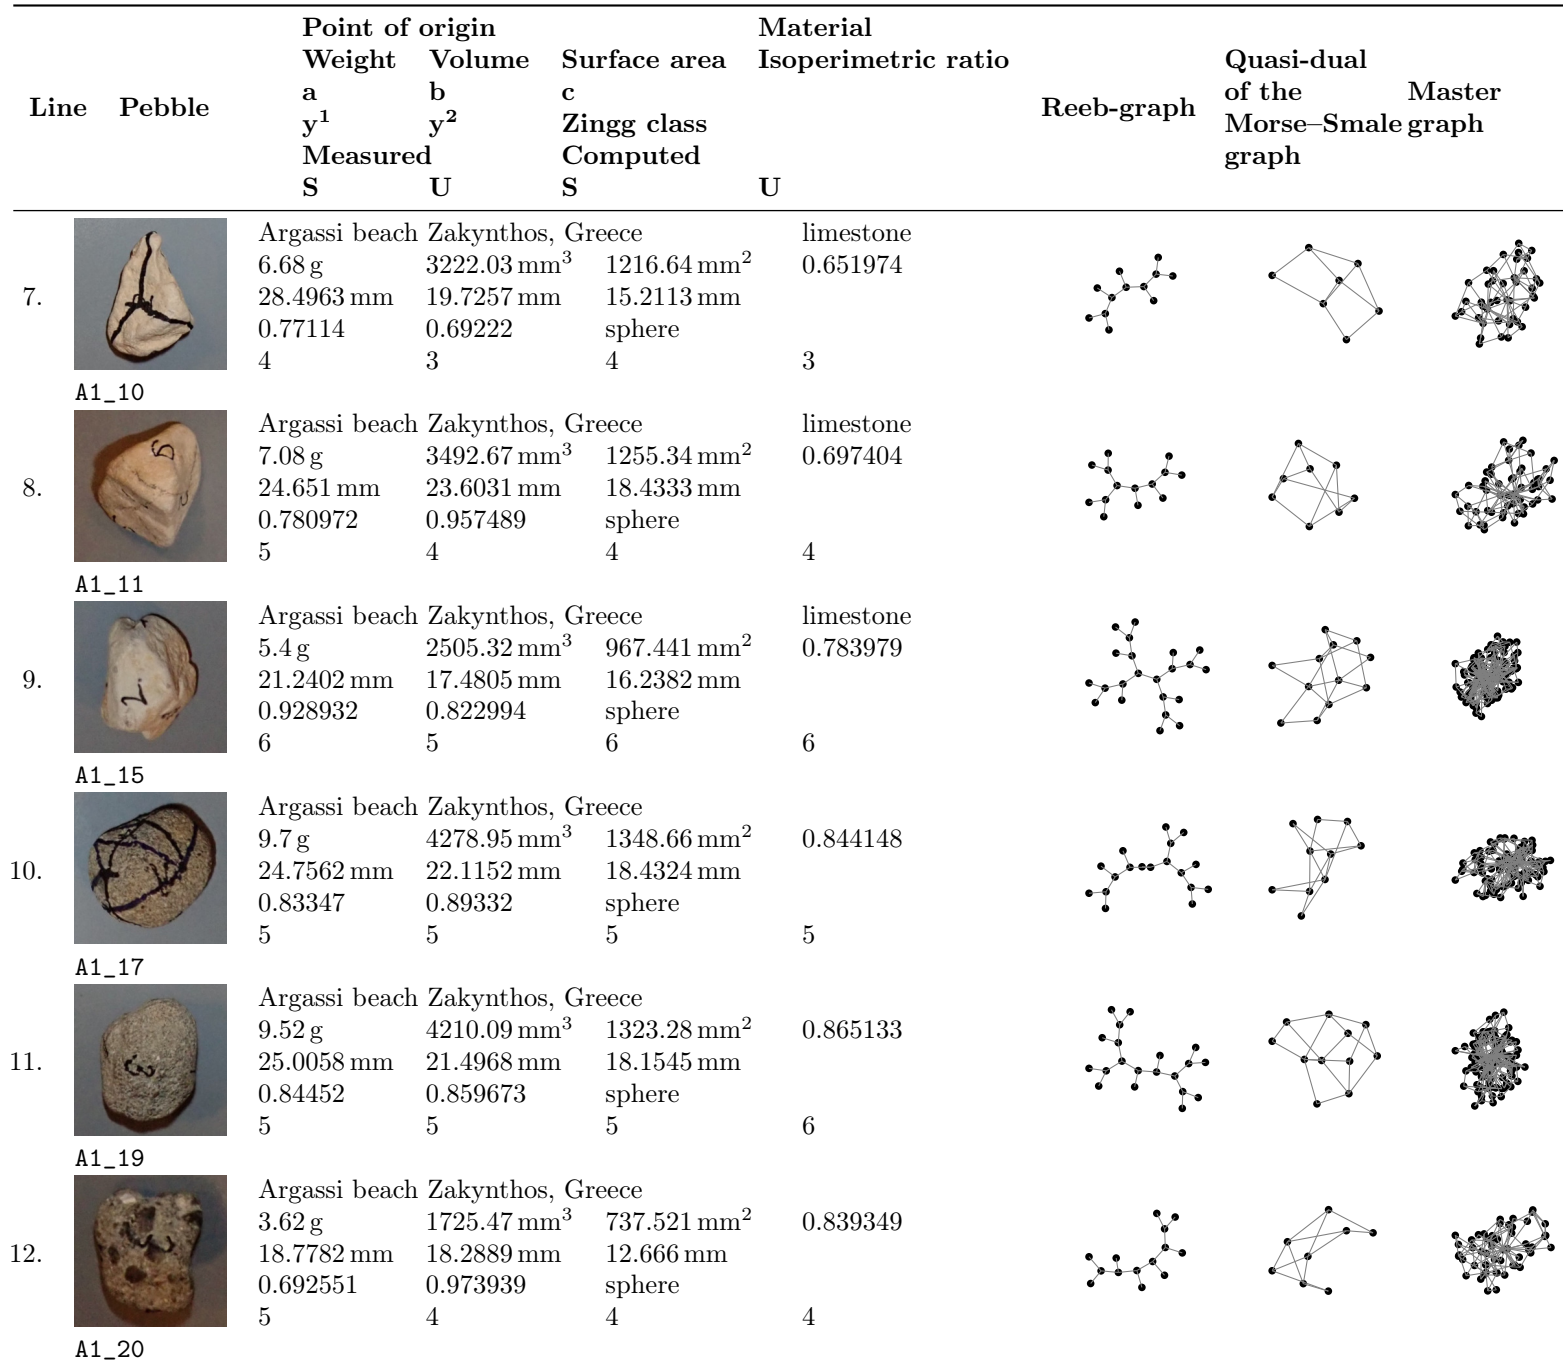 | Argassi beach<br>3.62 g<br>18.7782 mm<br>0.692551<br>5 | Zakynthos, Greece<br>1725.47 mm <sup>3</sup><br>18.2889 mm<br>0.973939<br>4 | 737.521 mm <sup>2</sup><br>12.666 mm<br>sphere<br>4  | 0.839349              | 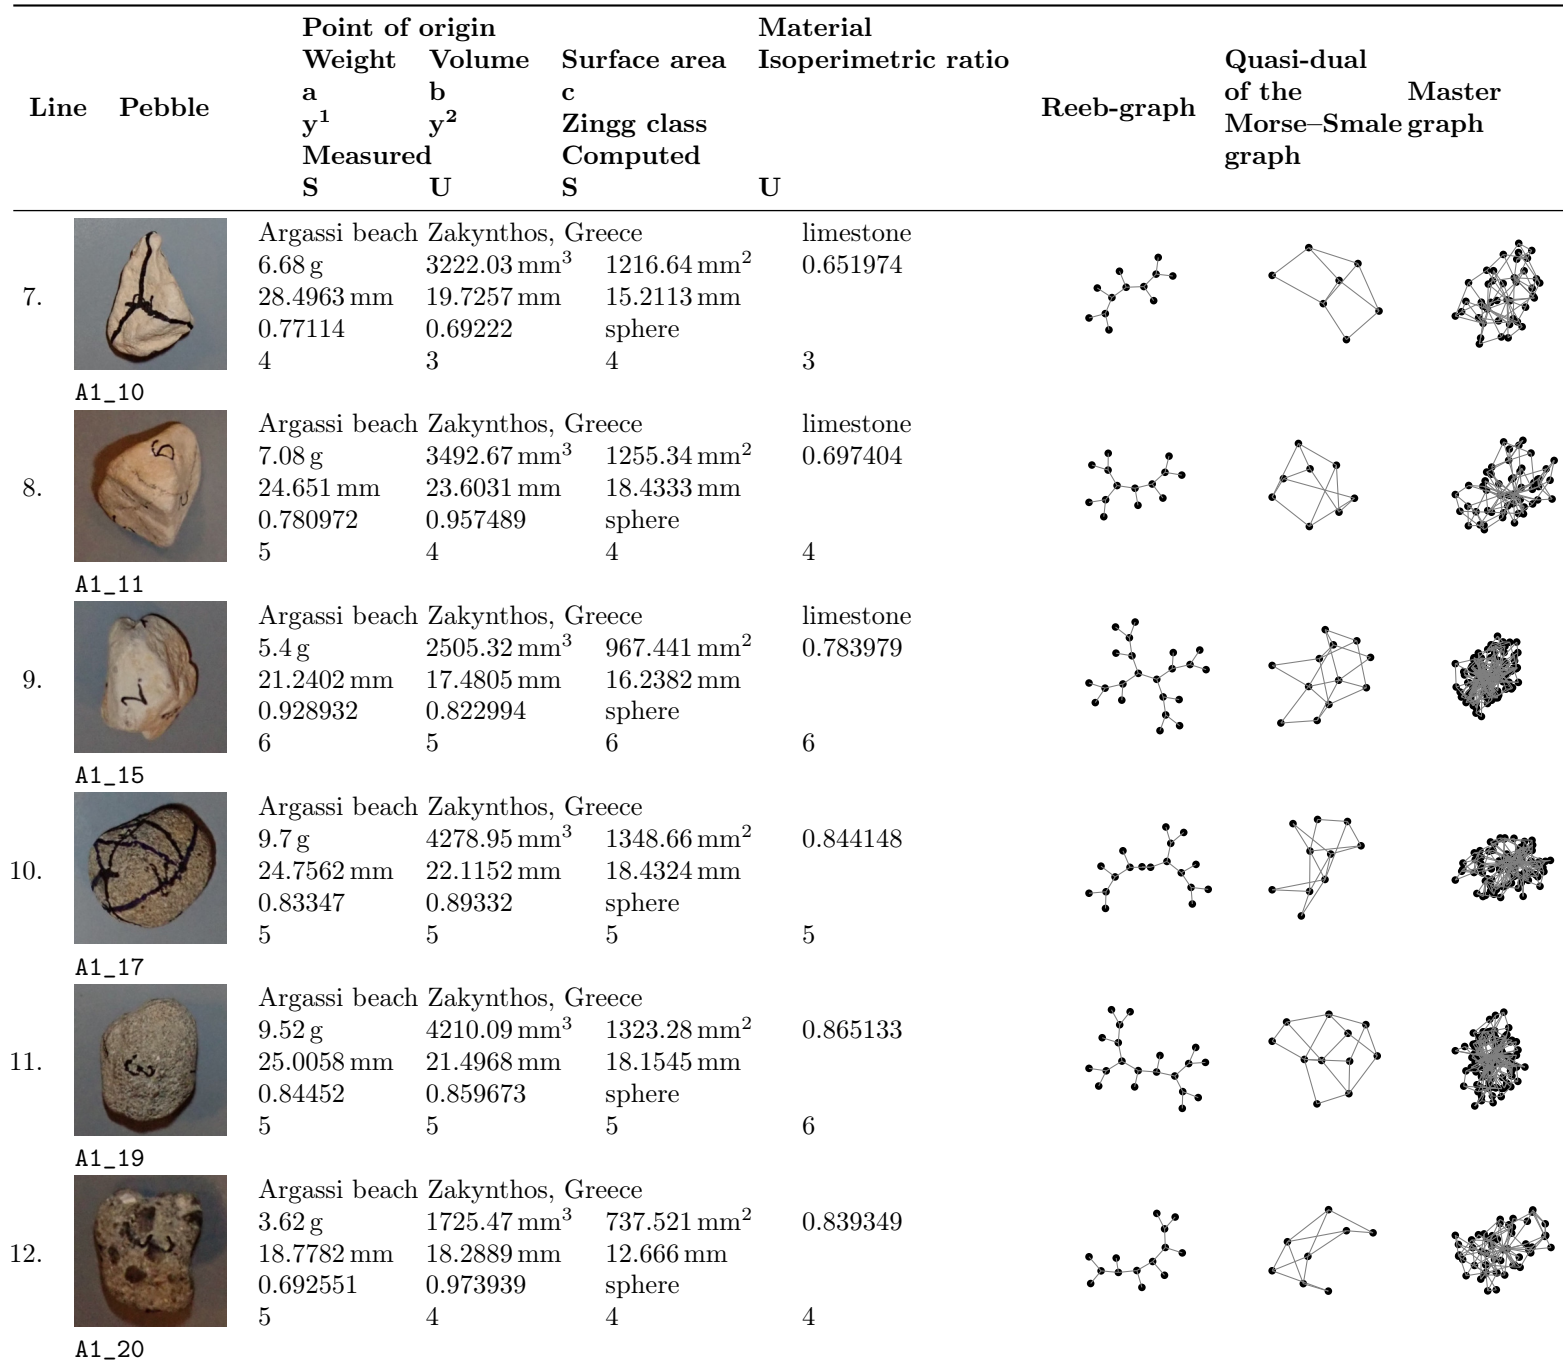 | 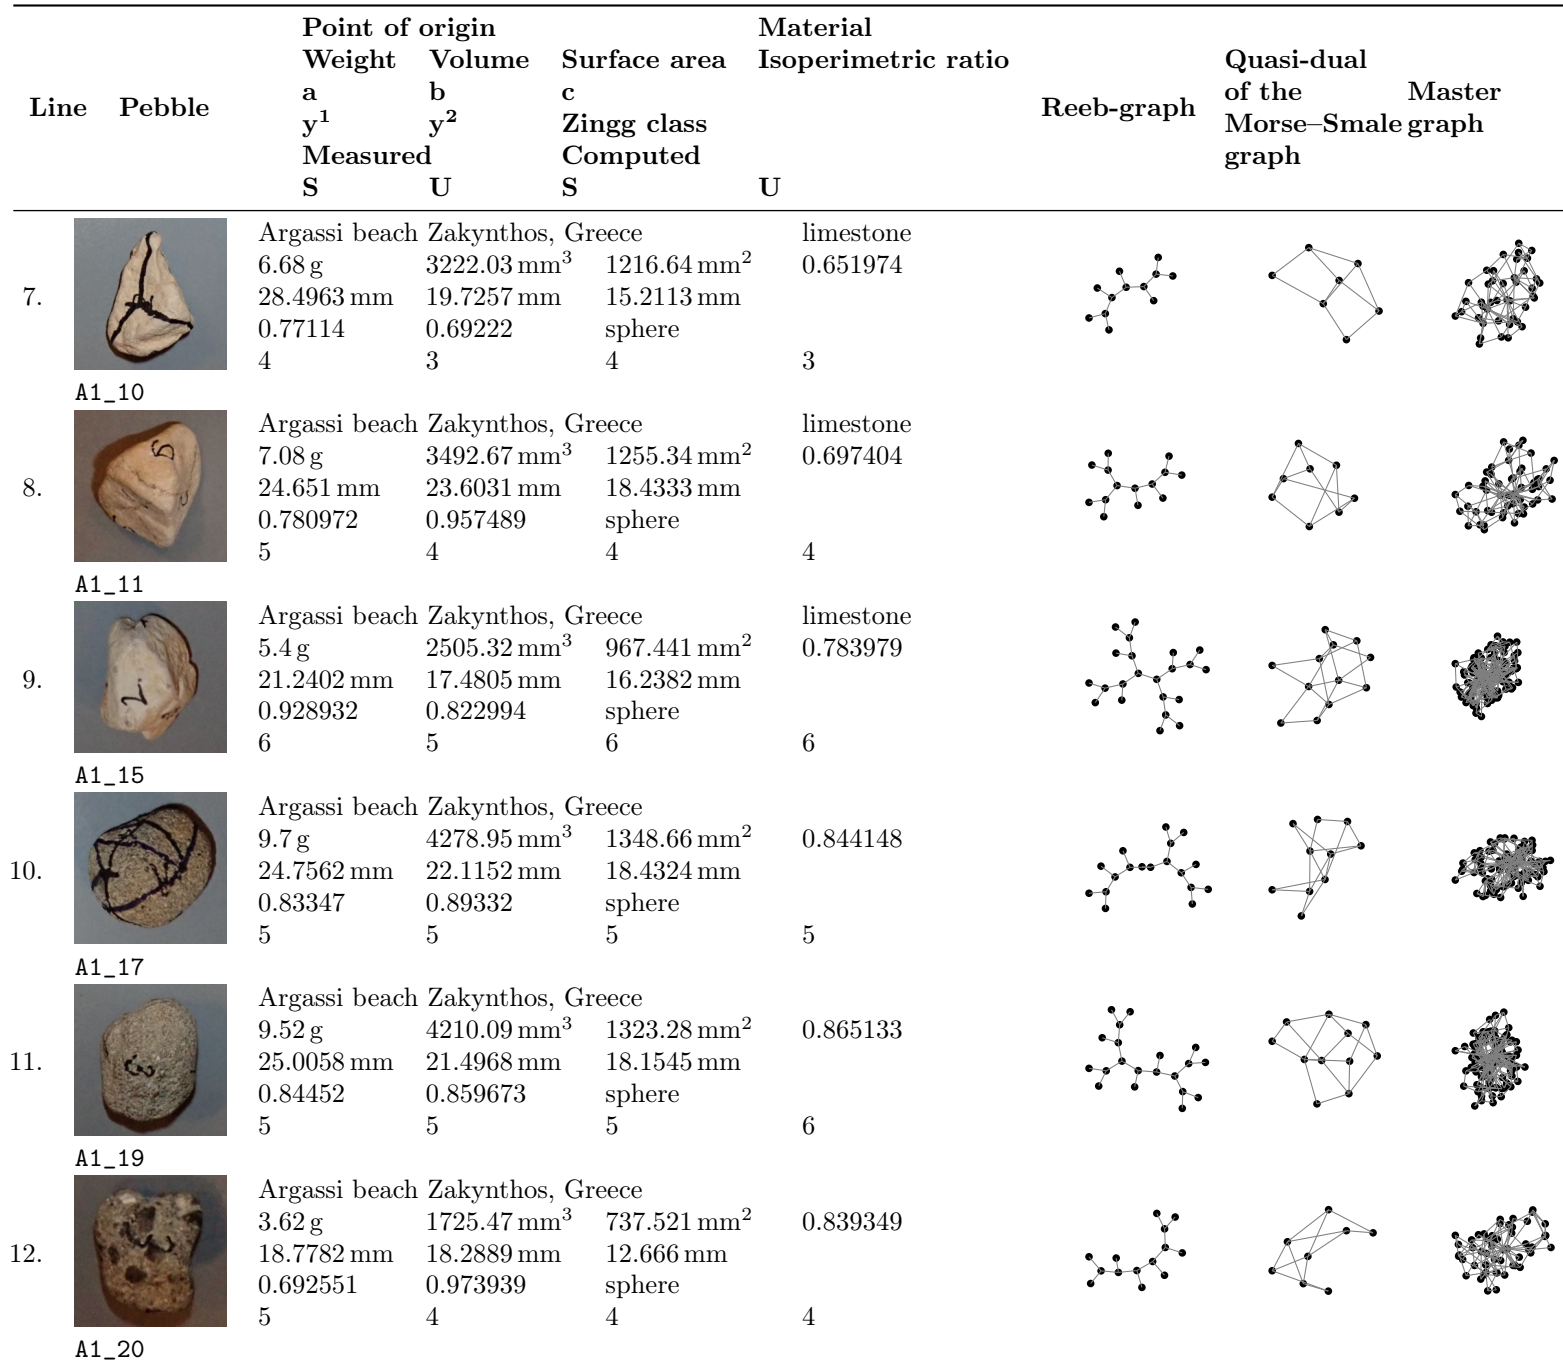 | 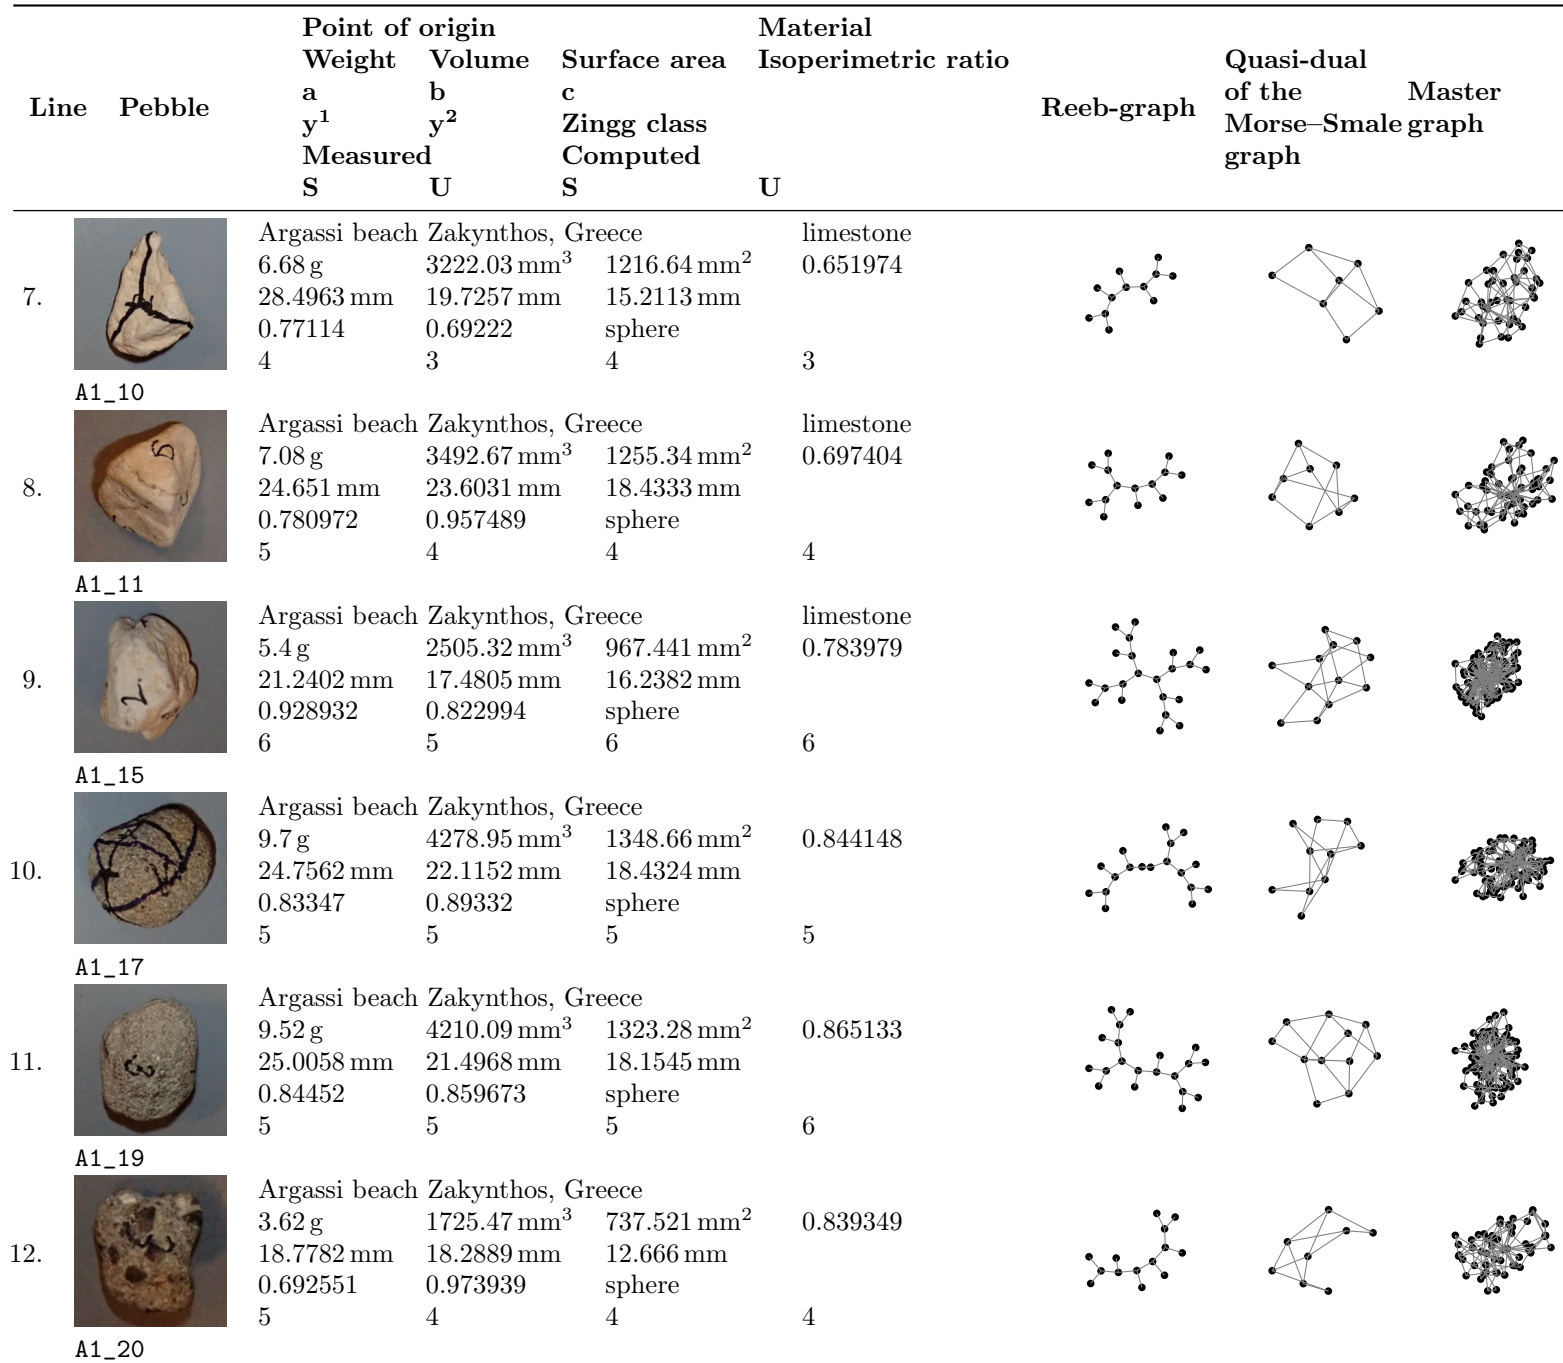 |
| A1_20 |                                                                                     |                                                        |                                                                             |                                                      |                       |                                                                                       |                                                                                       |                                                                                       |

| Line  | Pebble                                                                              | Point of origin                                         |                                                                             |                                                     | Material                       | Reeb-graph                                                                            | Quasi-dual<br>of the<br>Morse–Smale<br>graph                                          | Master                                                                                |
|-------|-------------------------------------------------------------------------------------|---------------------------------------------------------|-----------------------------------------------------------------------------|-----------------------------------------------------|--------------------------------|---------------------------------------------------------------------------------------|---------------------------------------------------------------------------------------|---------------------------------------------------------------------------------------|
|       |                                                                                     | Weight                                                  | Volume                                                                      | Surface area                                        |                                |                                                                                       |                                                                                       |                                                                                       |
|       |                                                                                     | a                                                       | b                                                                           | c                                                   |                                |                                                                                       |                                                                                       |                                                                                       |
|       |                                                                                     | y <sup>1</sup><br>Measured<br>S                         | y <sup>2</sup><br>U                                                         | Zingg class<br>Computed<br>S                        |                                |                                                                                       |                                                                                       |                                                                                       |
| 13.   | 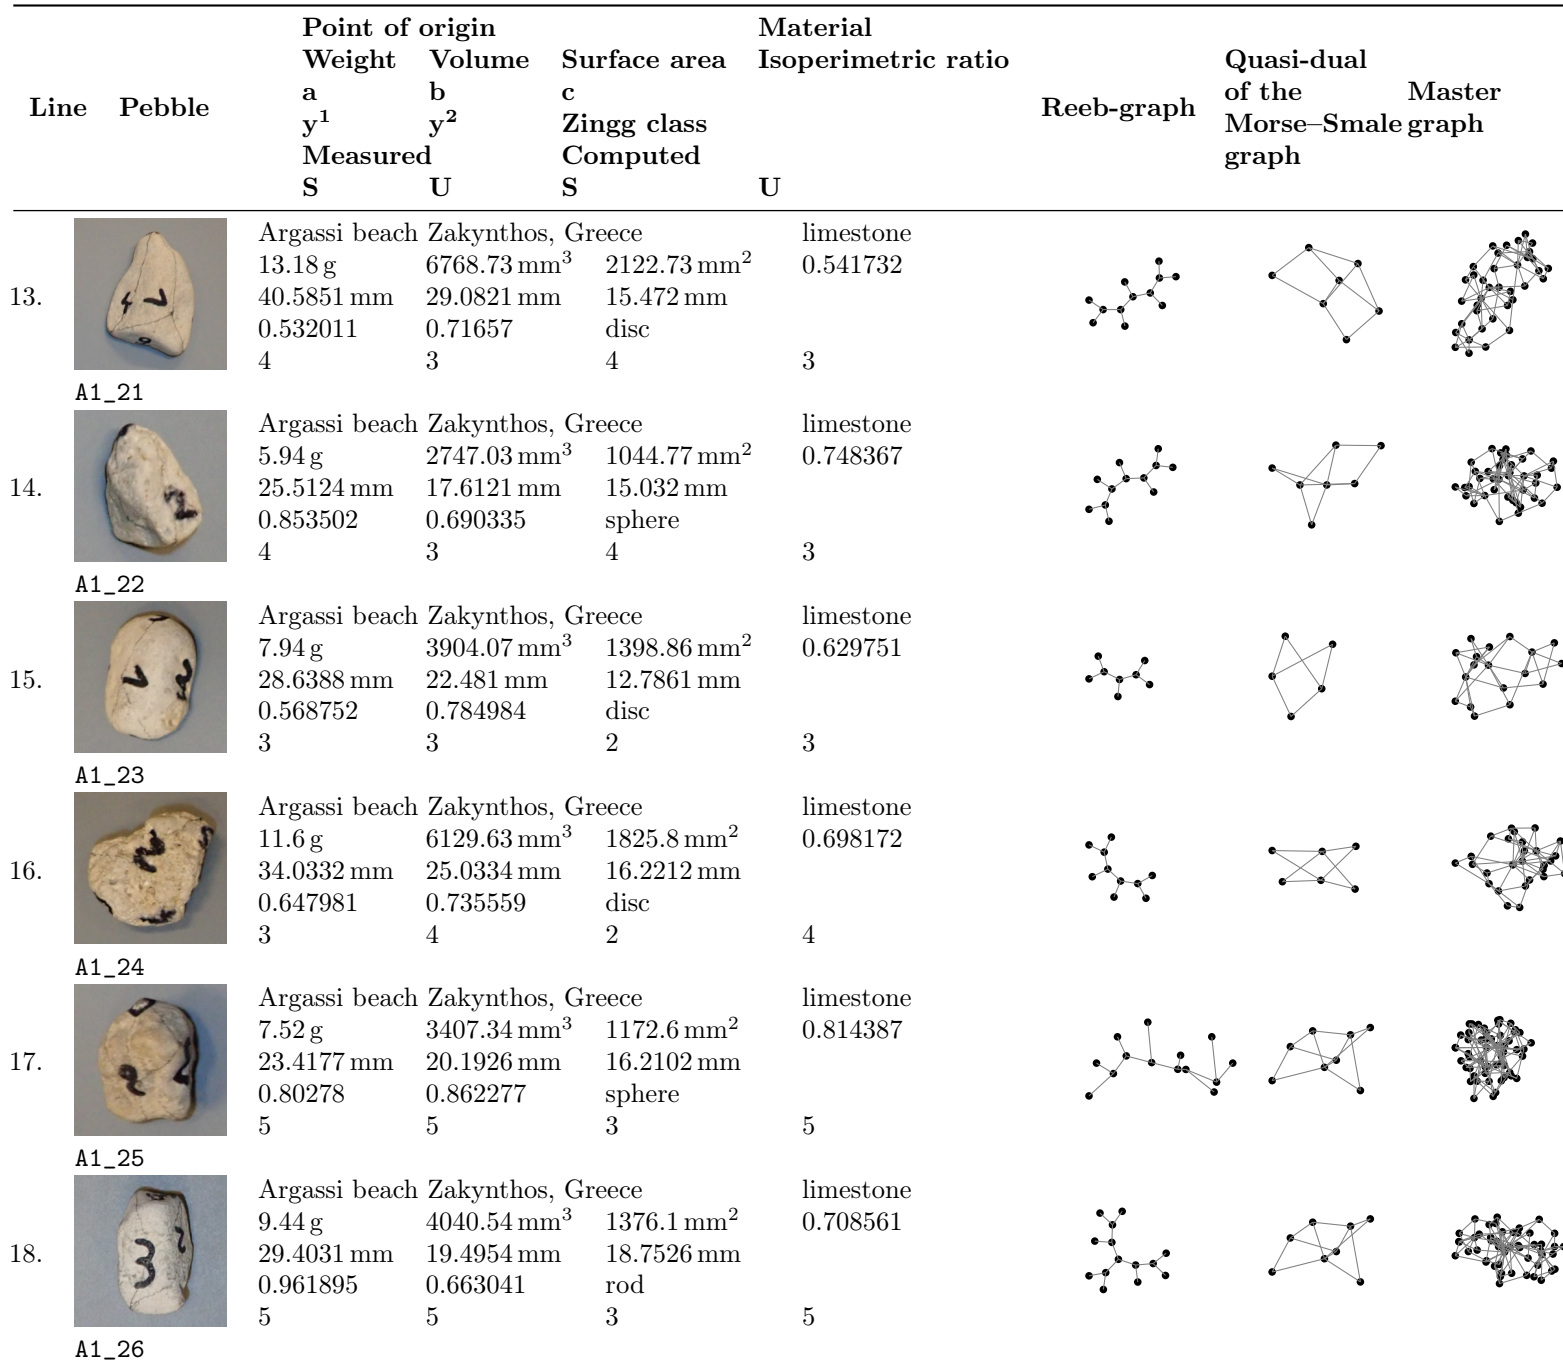   | Argassi beach<br>13.18 g<br>40.5851 mm<br>0.532011<br>4 | Zakynthos, Greece<br>6768.73 mm <sup>3</sup><br>29.0821 mm<br>0.71657<br>3  | 1222.73 mm <sup>2</sup><br>15.472 mm<br>disc<br>4   | limestone<br>0.541732<br><br>3 | 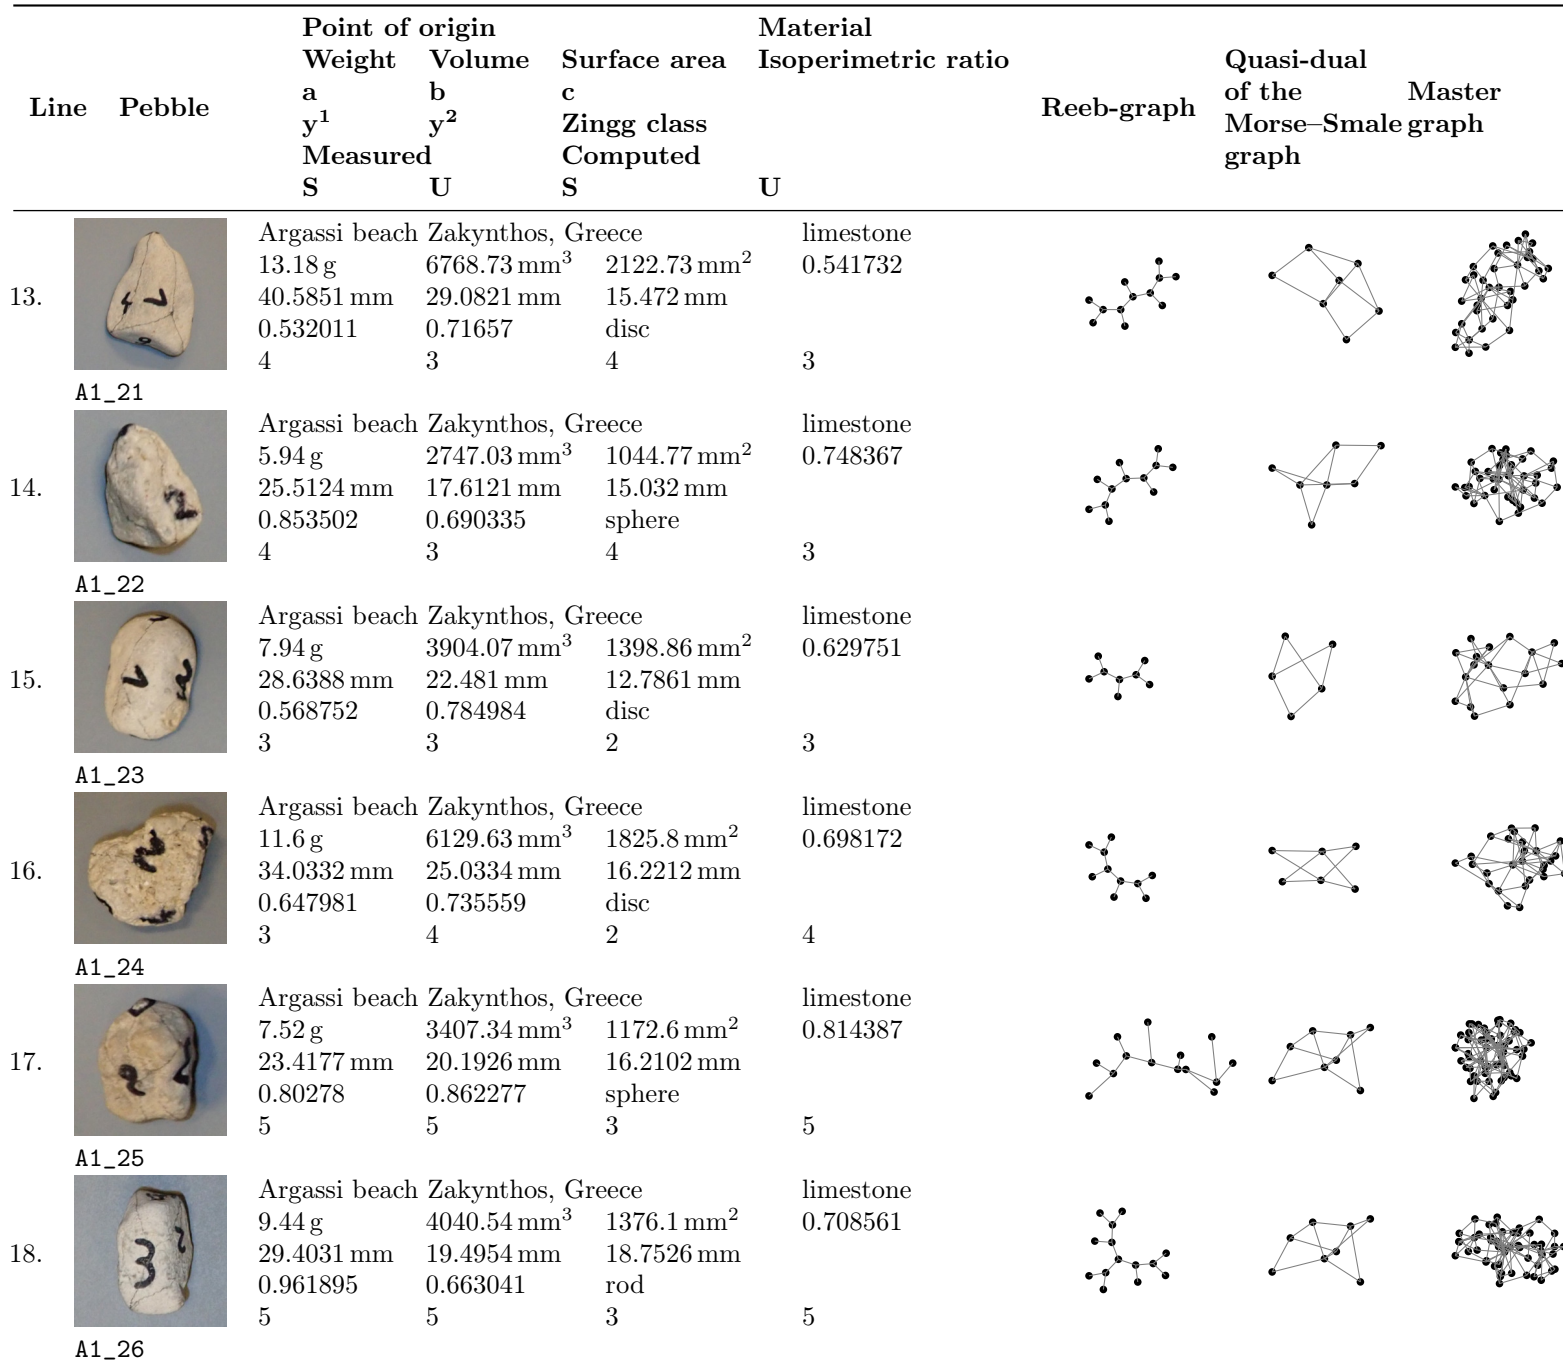   | 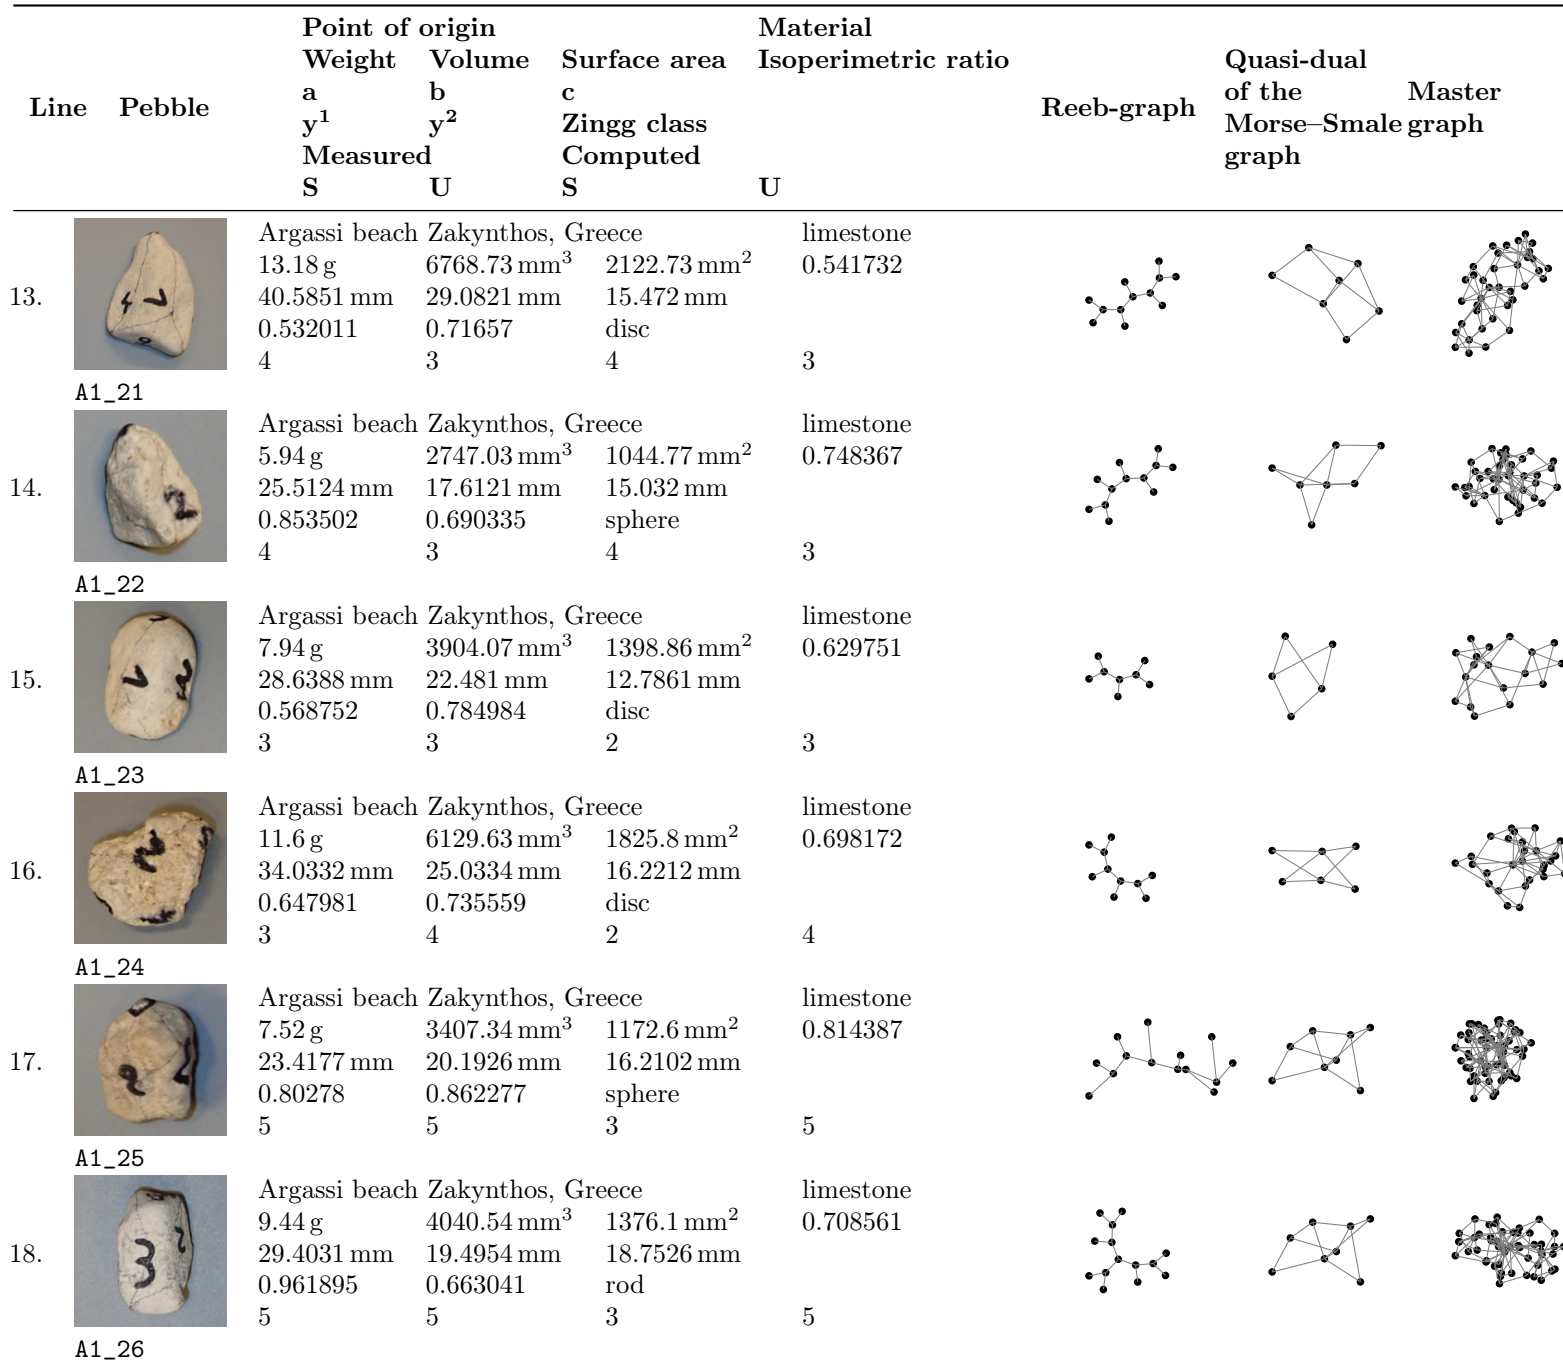   | 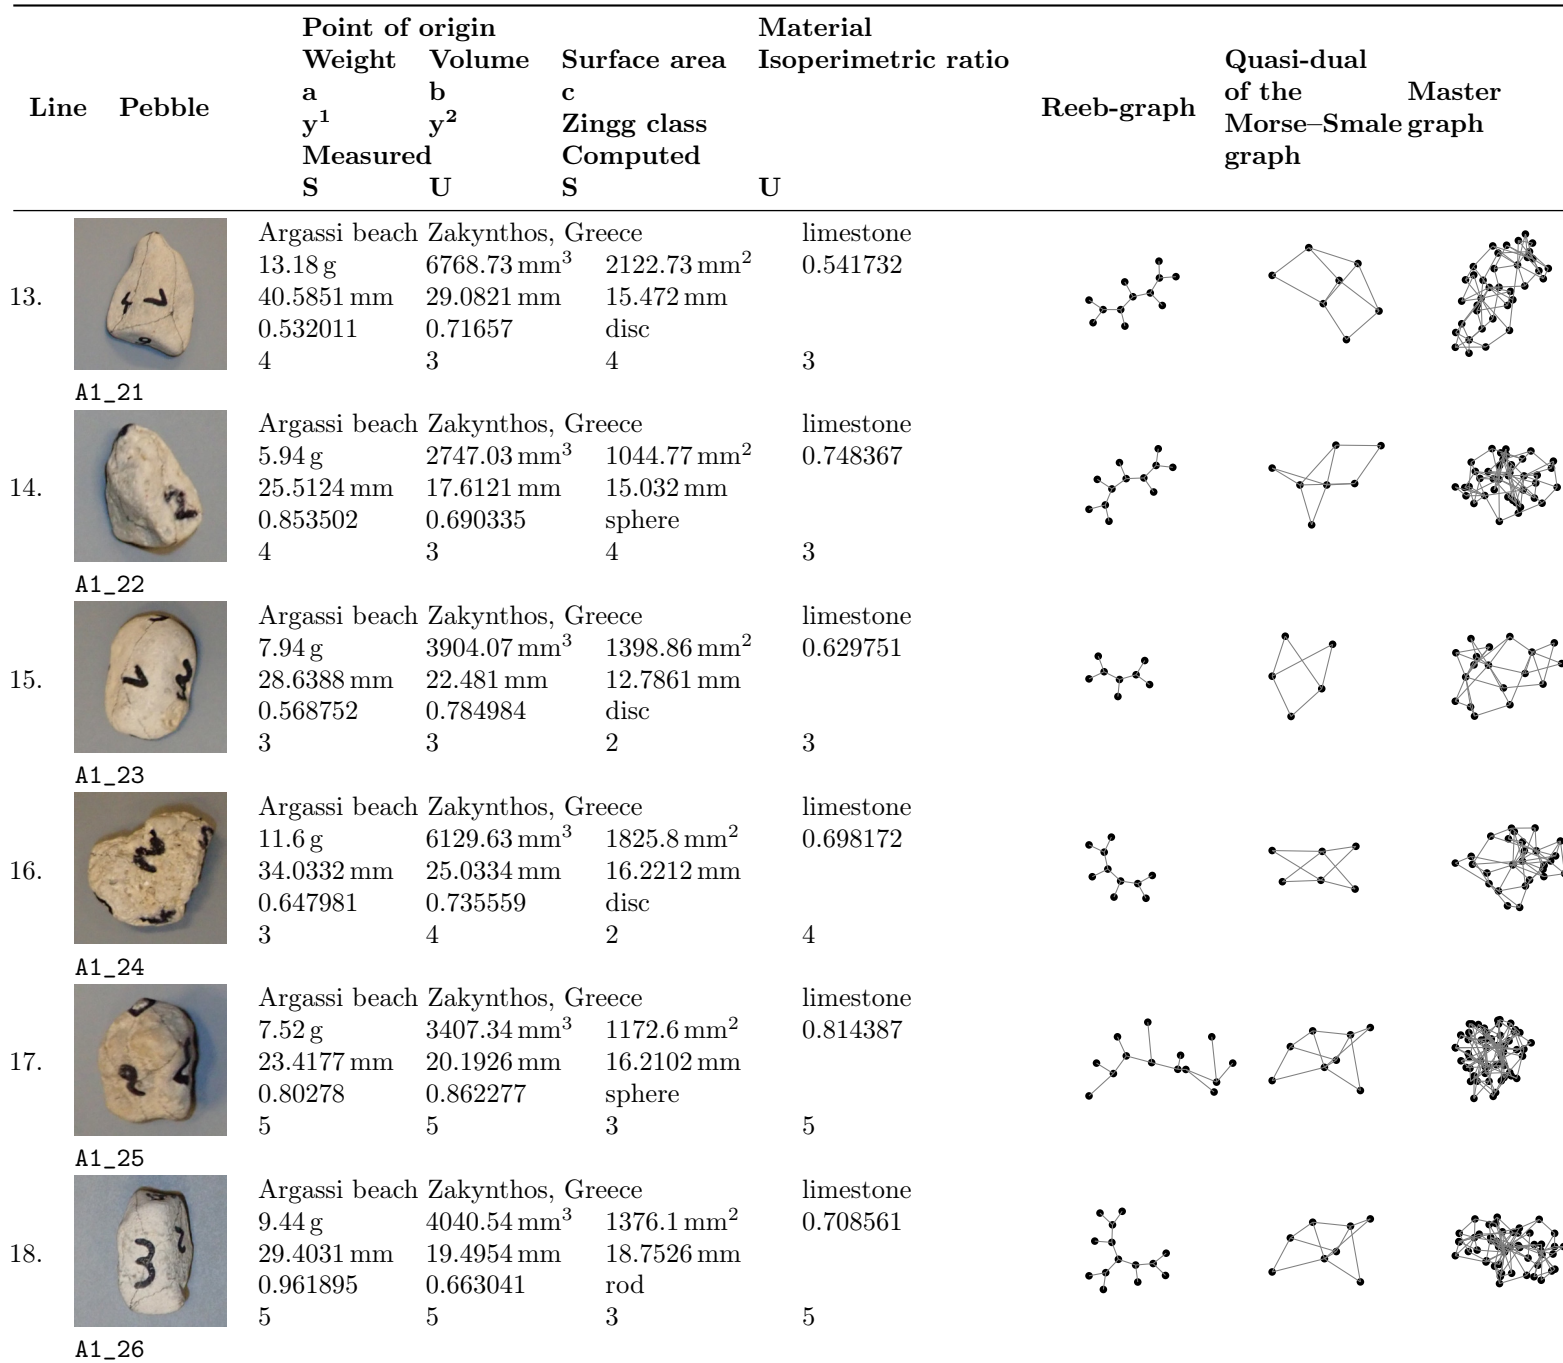   |
| A1_21 |                                                                                     |                                                         |                                                                             |                                                     |                                |                                                                                       |                                                                                       |                                                                                       |
| 14.   | 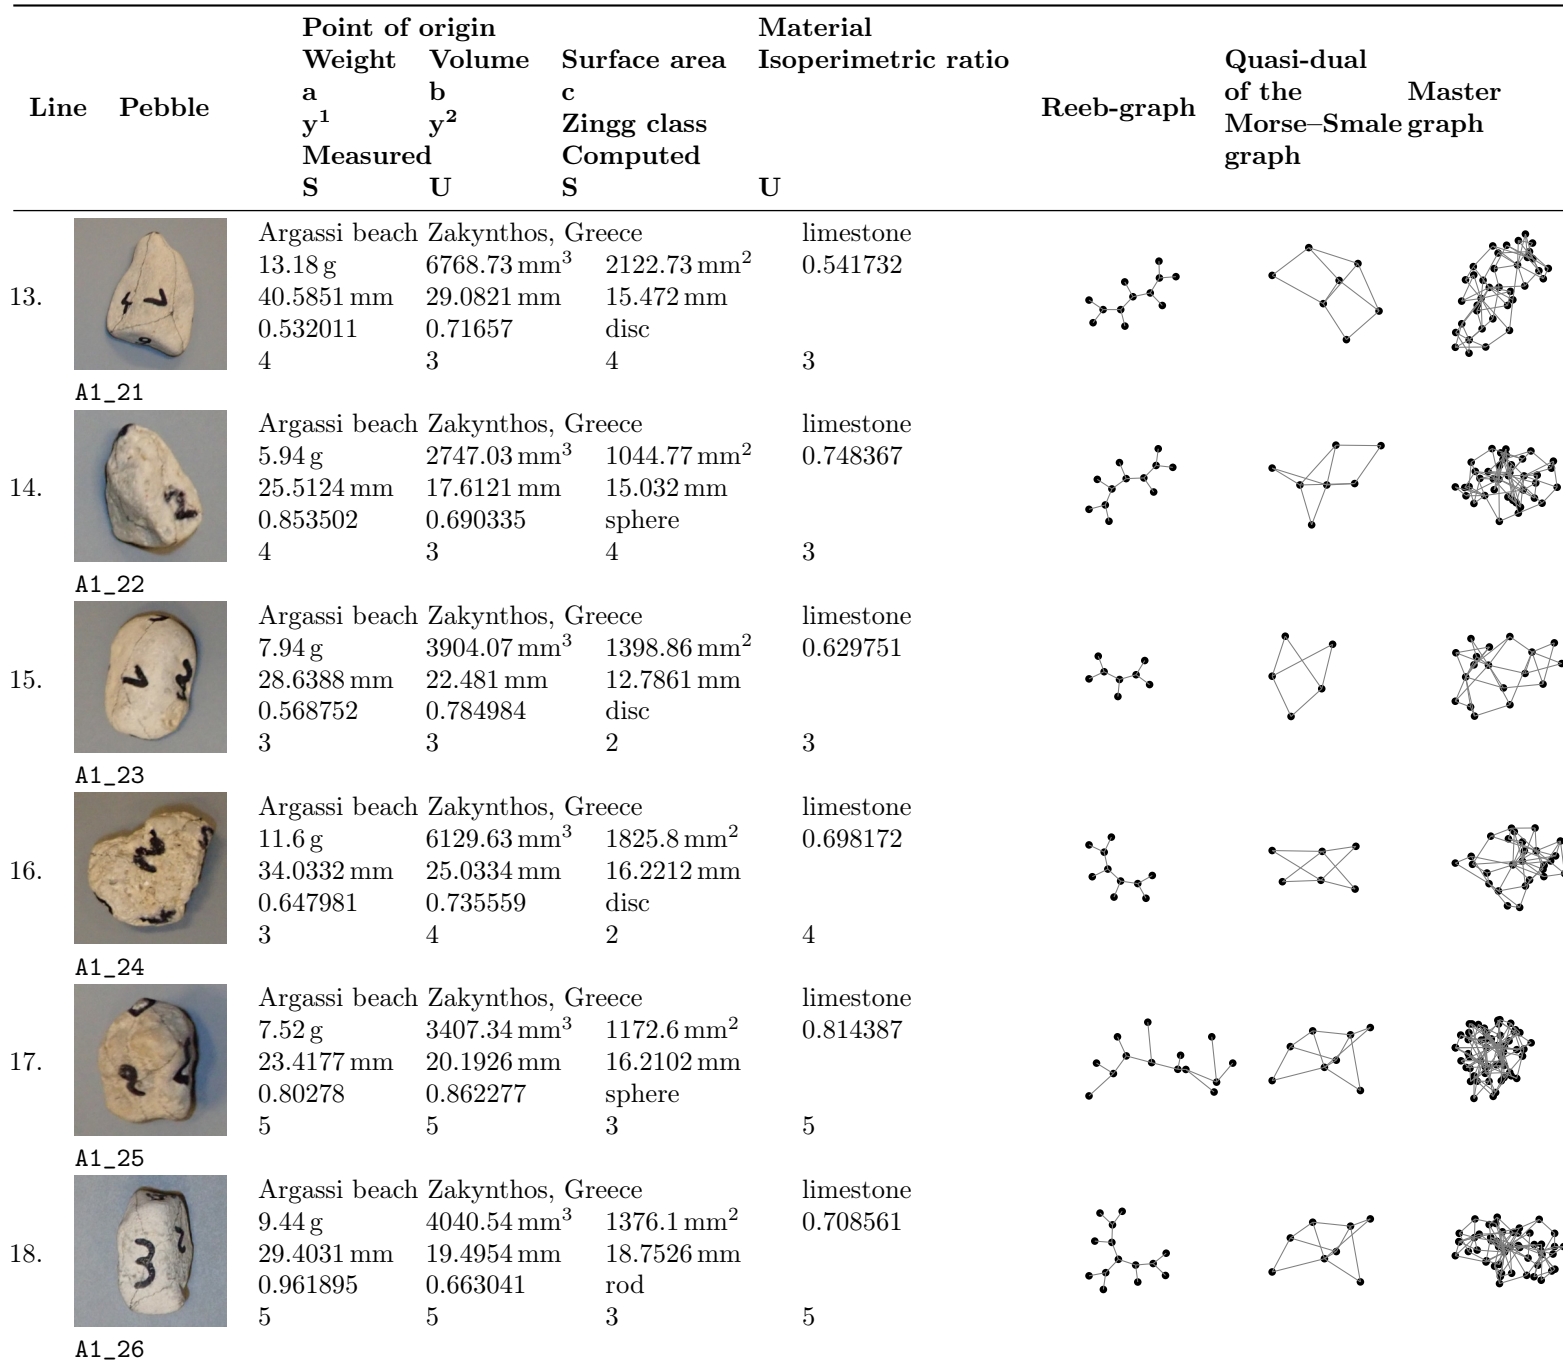   | Argassi beach<br>5.94 g<br>25.5124 mm<br>0.853502<br>4  | Zakynthos, Greece<br>2747.03 mm <sup>3</sup><br>17.6121 mm<br>0.690335<br>3 | 1044.77 mm <sup>2</sup><br>15.032 mm<br>sphere<br>4 | limestone<br>0.748367<br><br>3 | 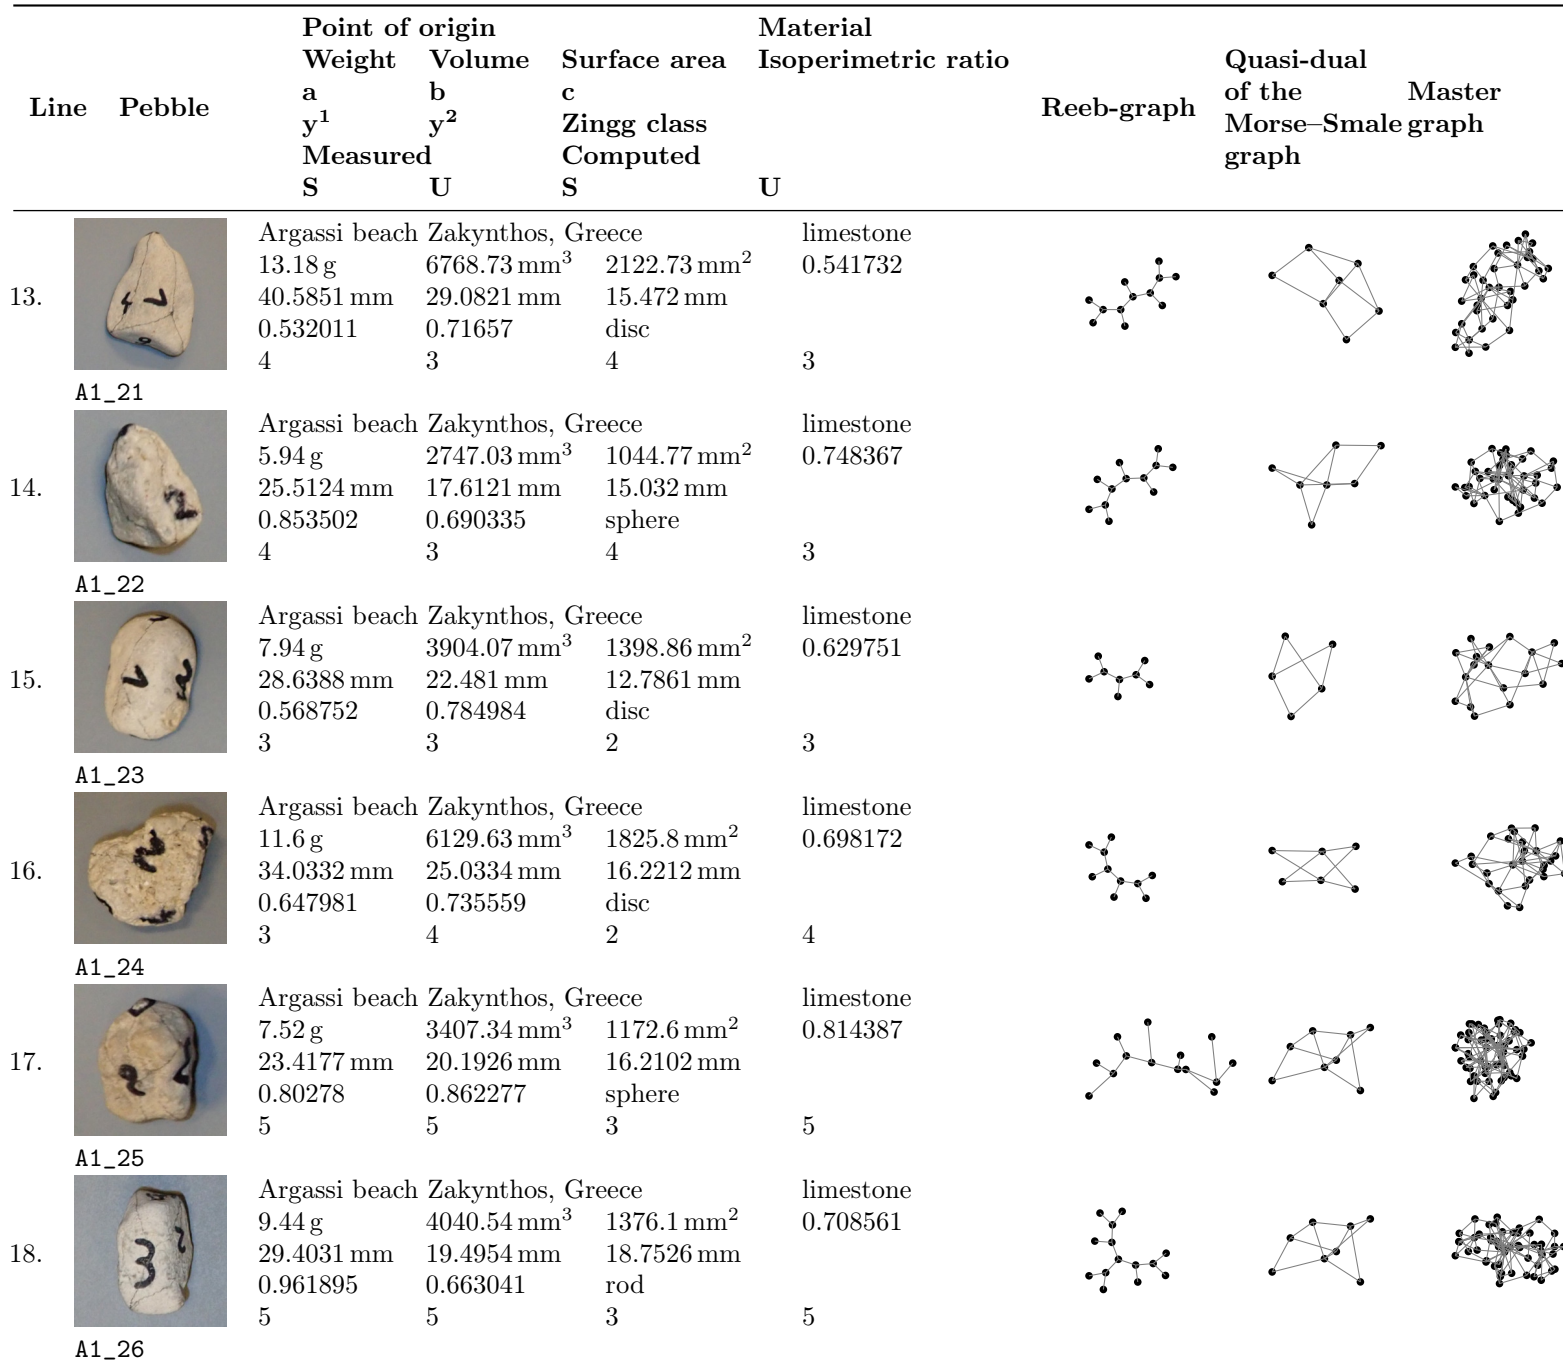   | 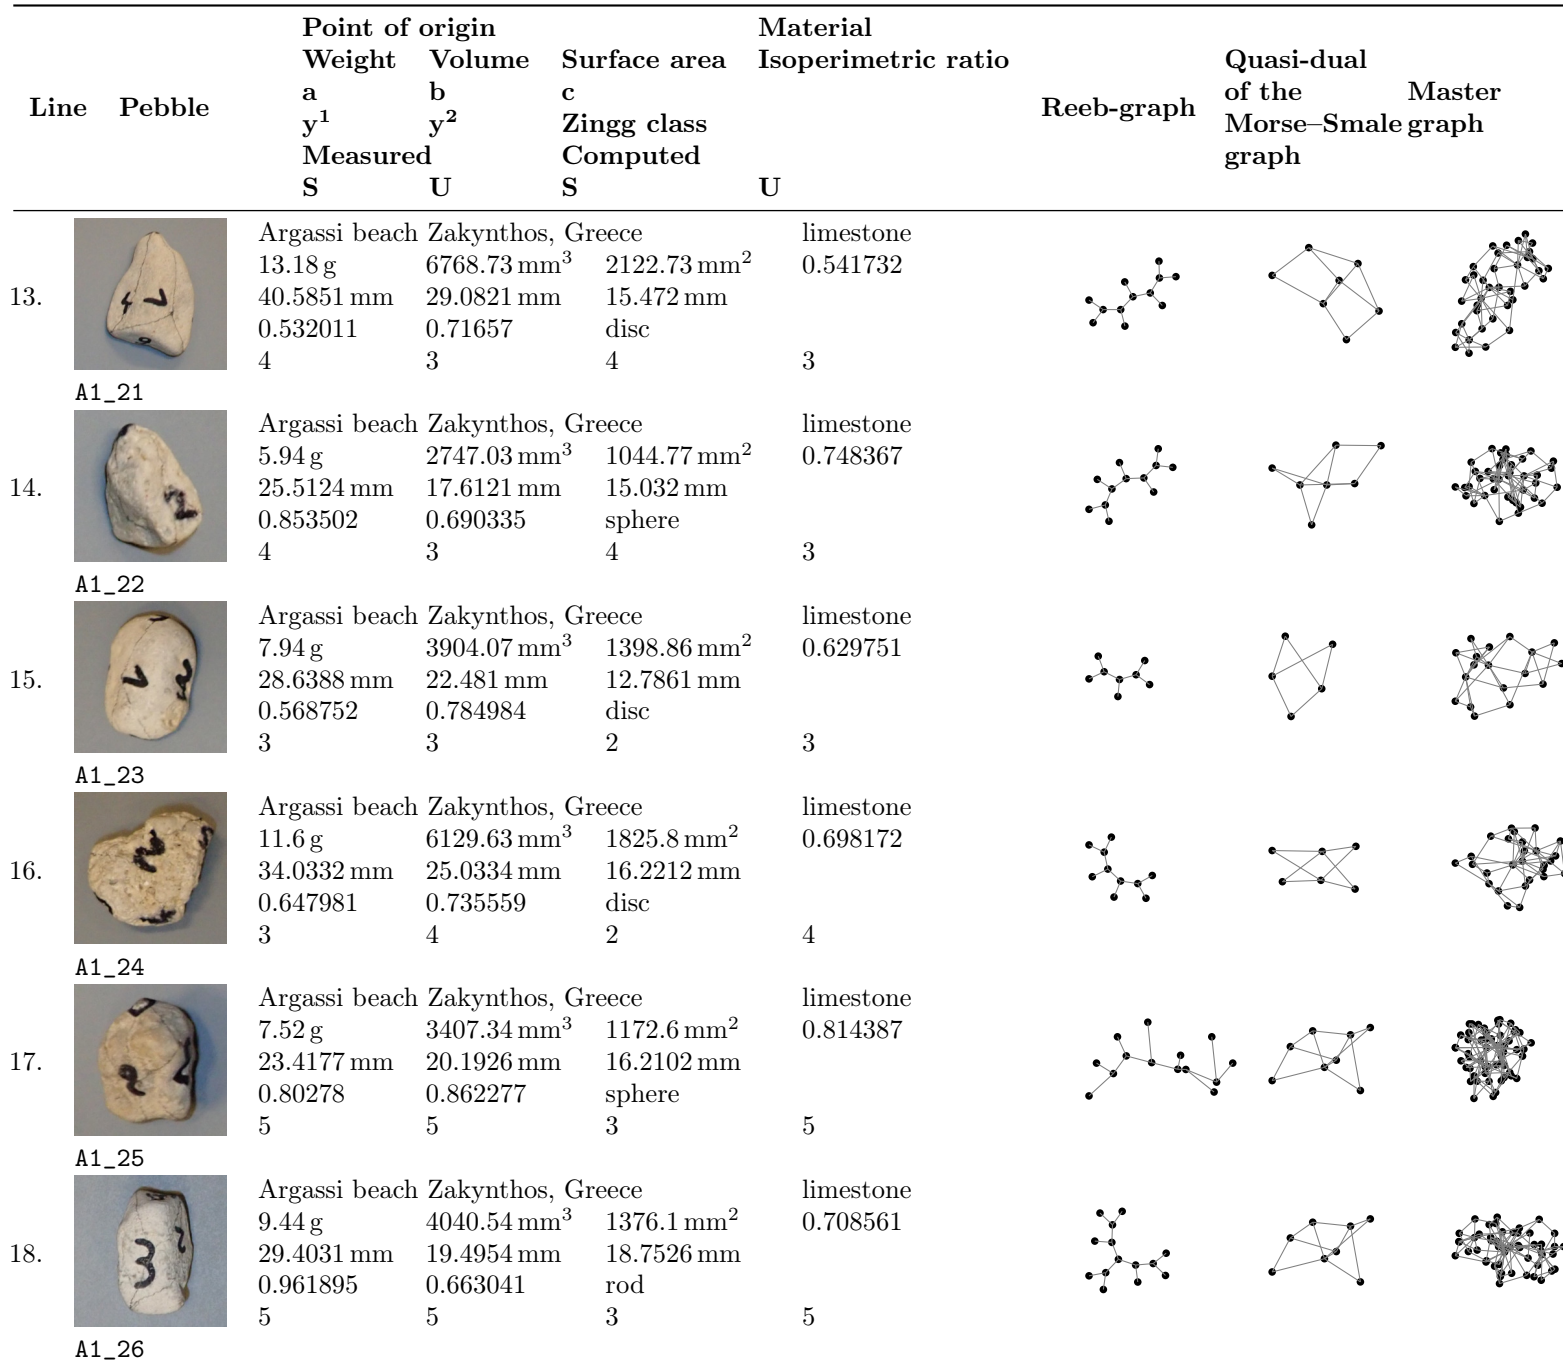   | 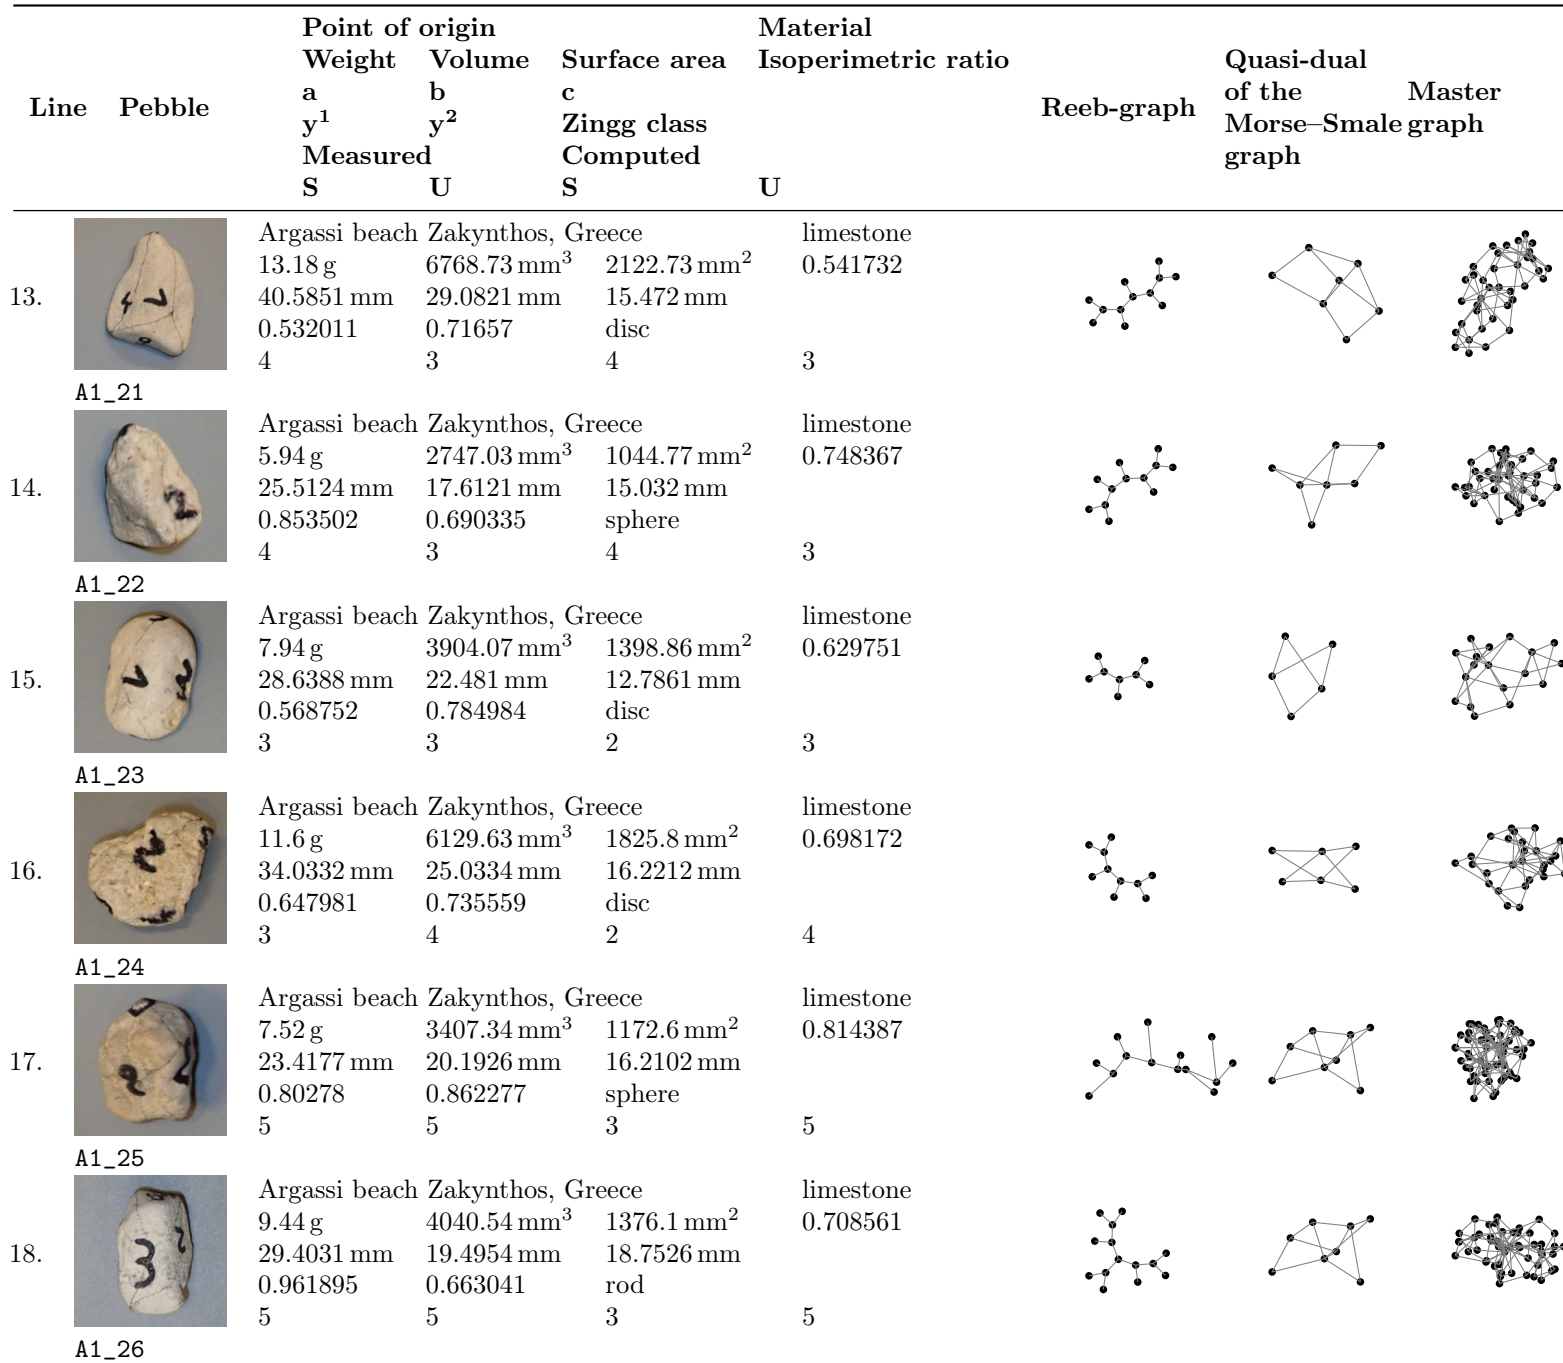   |
| A1_22 |                                                                                     |                                                         |                                                                             |                                                     |                                |                                                                                       |                                                                                       |                                                                                       |
| 15.   | 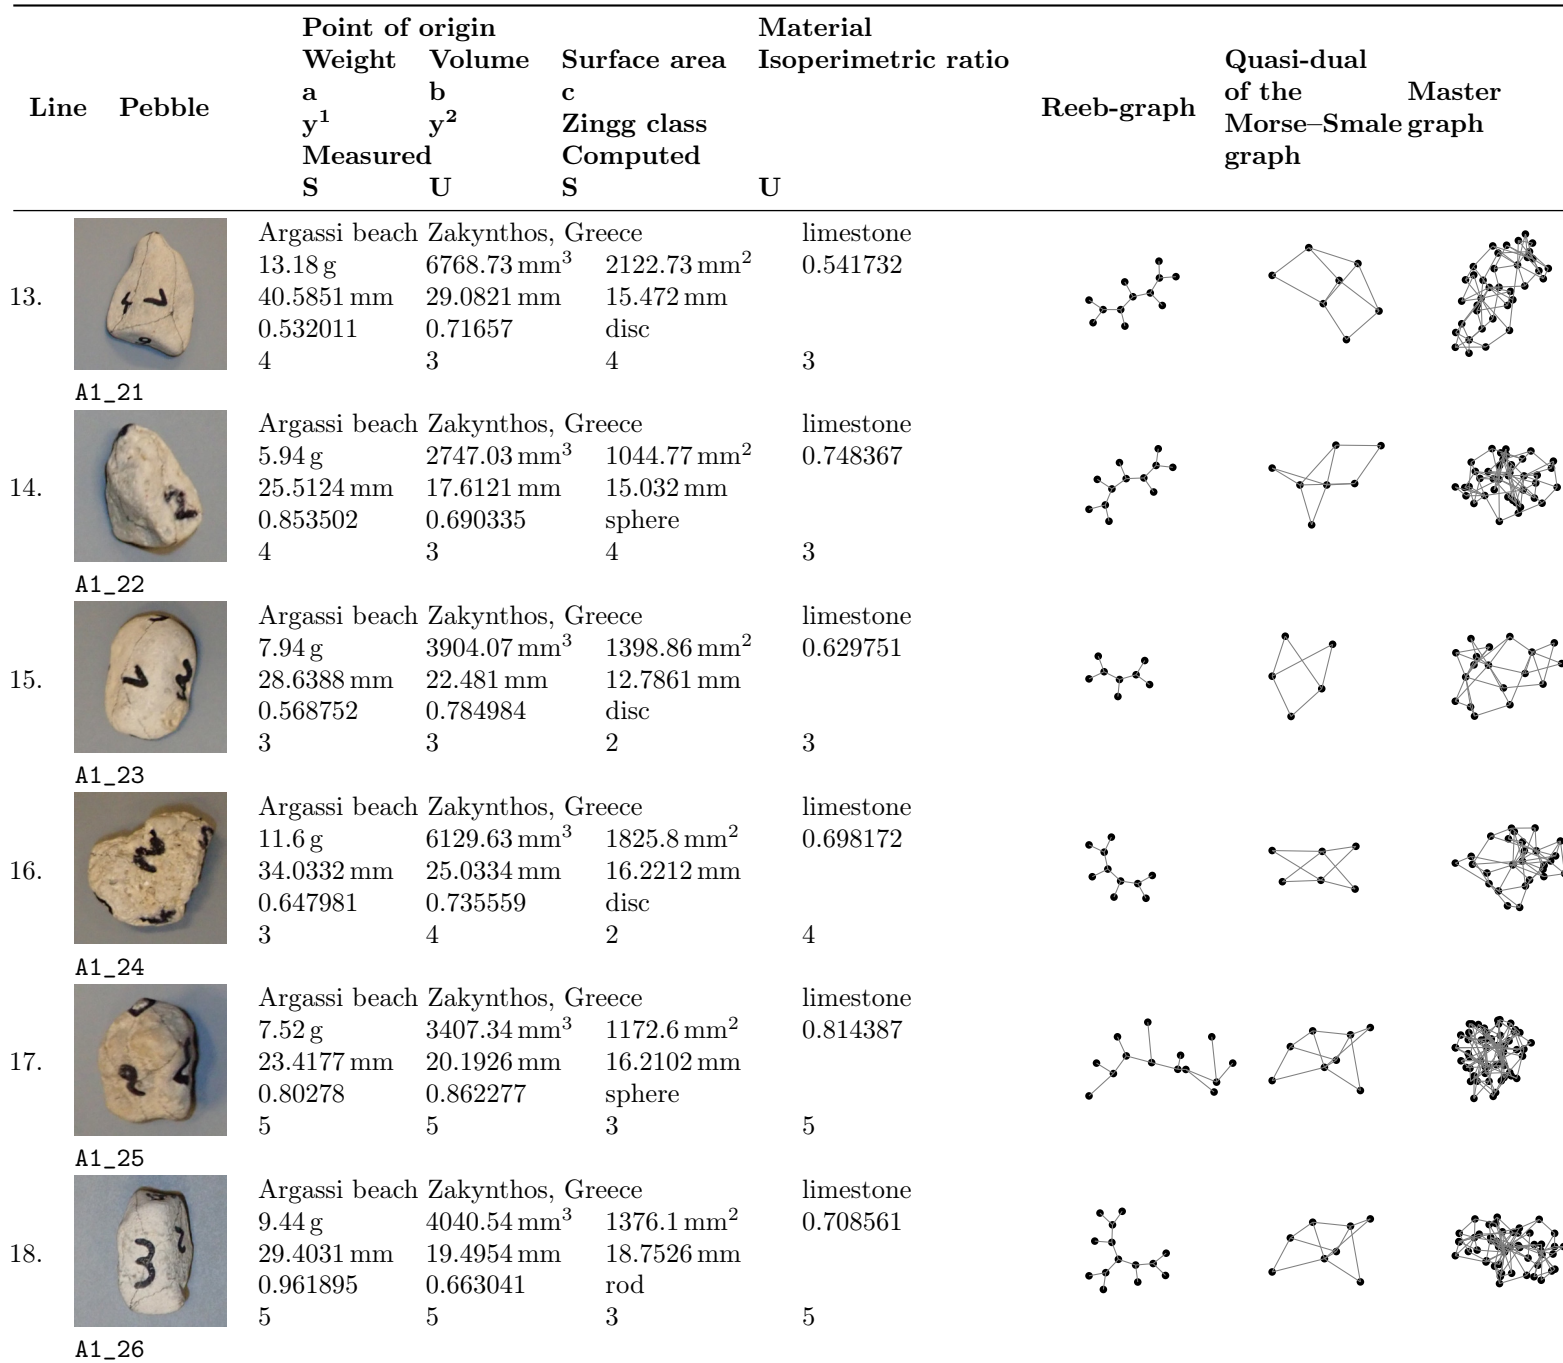   | Argassi beach<br>7.94 g<br>28.6388 mm<br>0.568752<br>3  | Zakynthos, Greece<br>3904.07 mm <sup>3</sup><br>22.481 mm<br>0.784984<br>3  | 1398.86 mm <sup>2</sup><br>12.7861 mm<br>disc<br>2  | limestone<br>0.629751<br><br>3 | 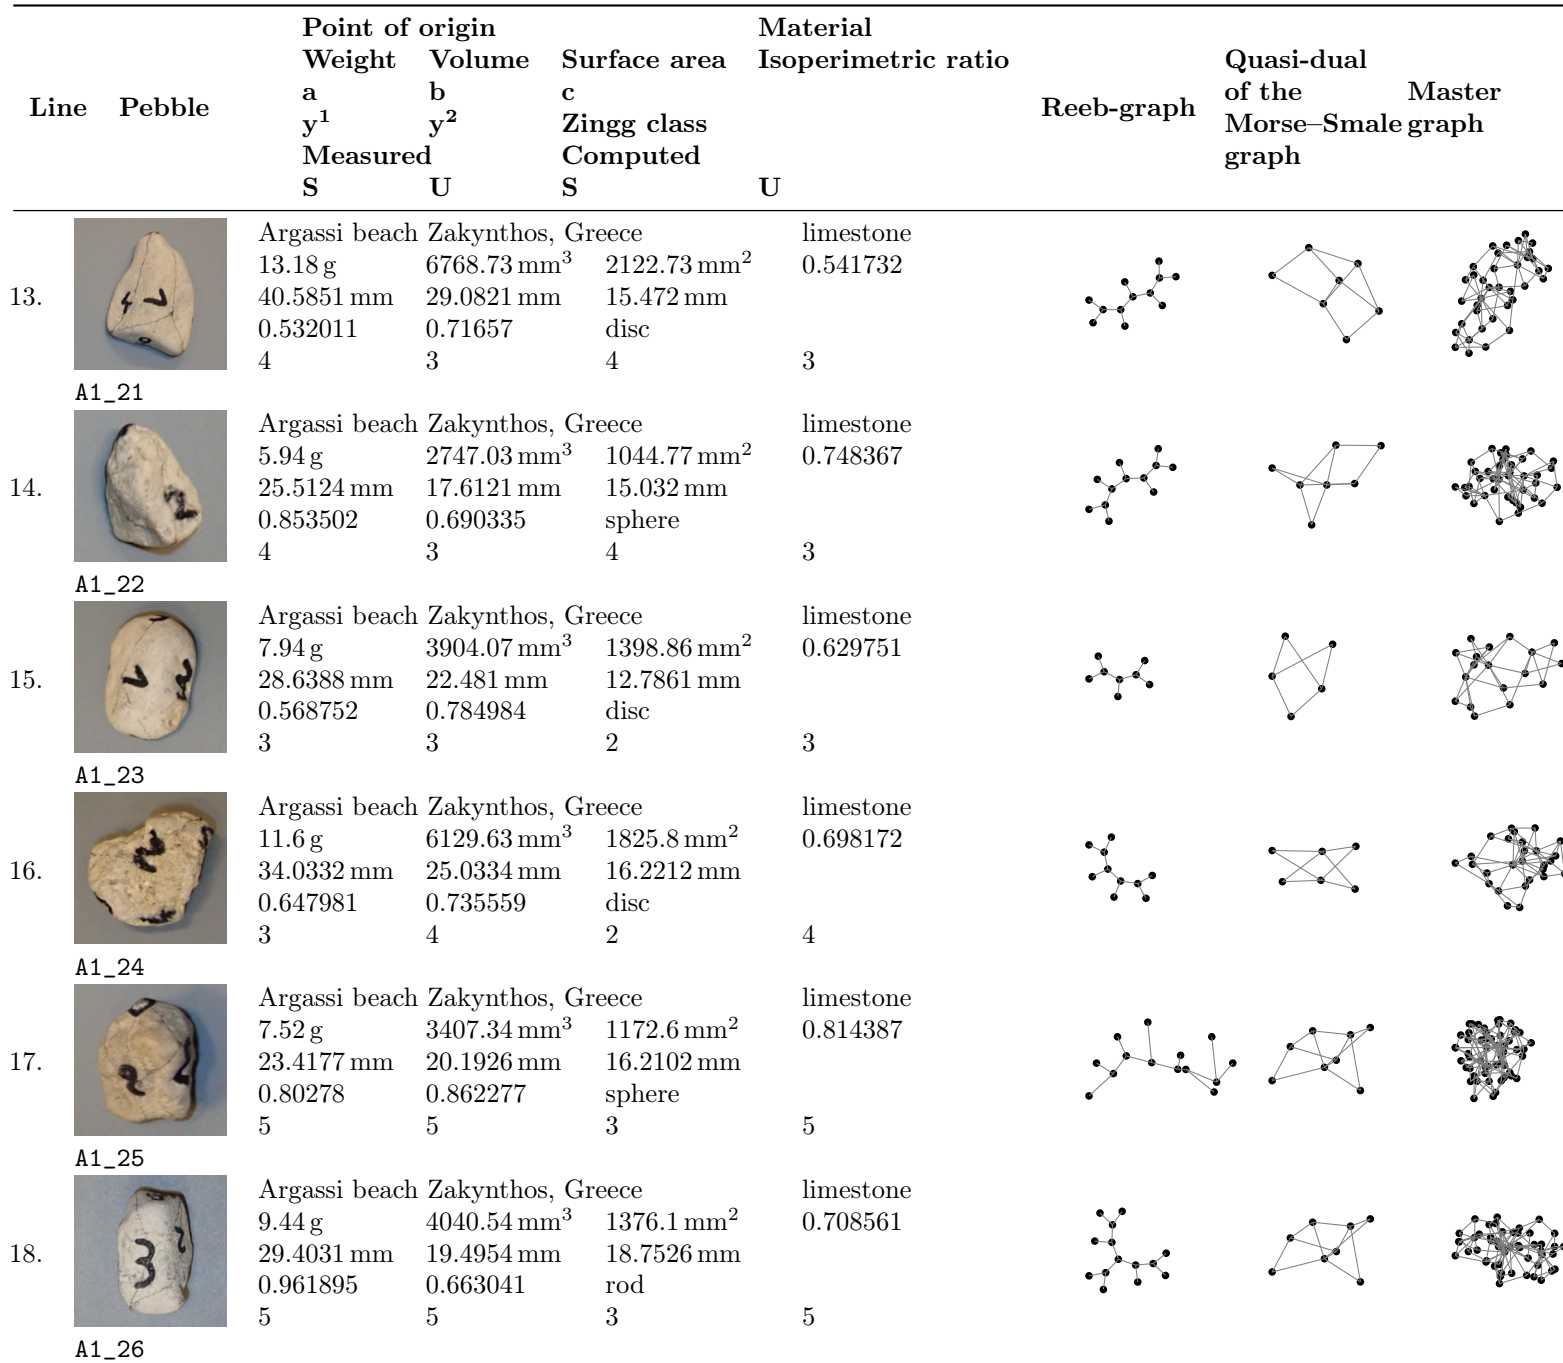   | 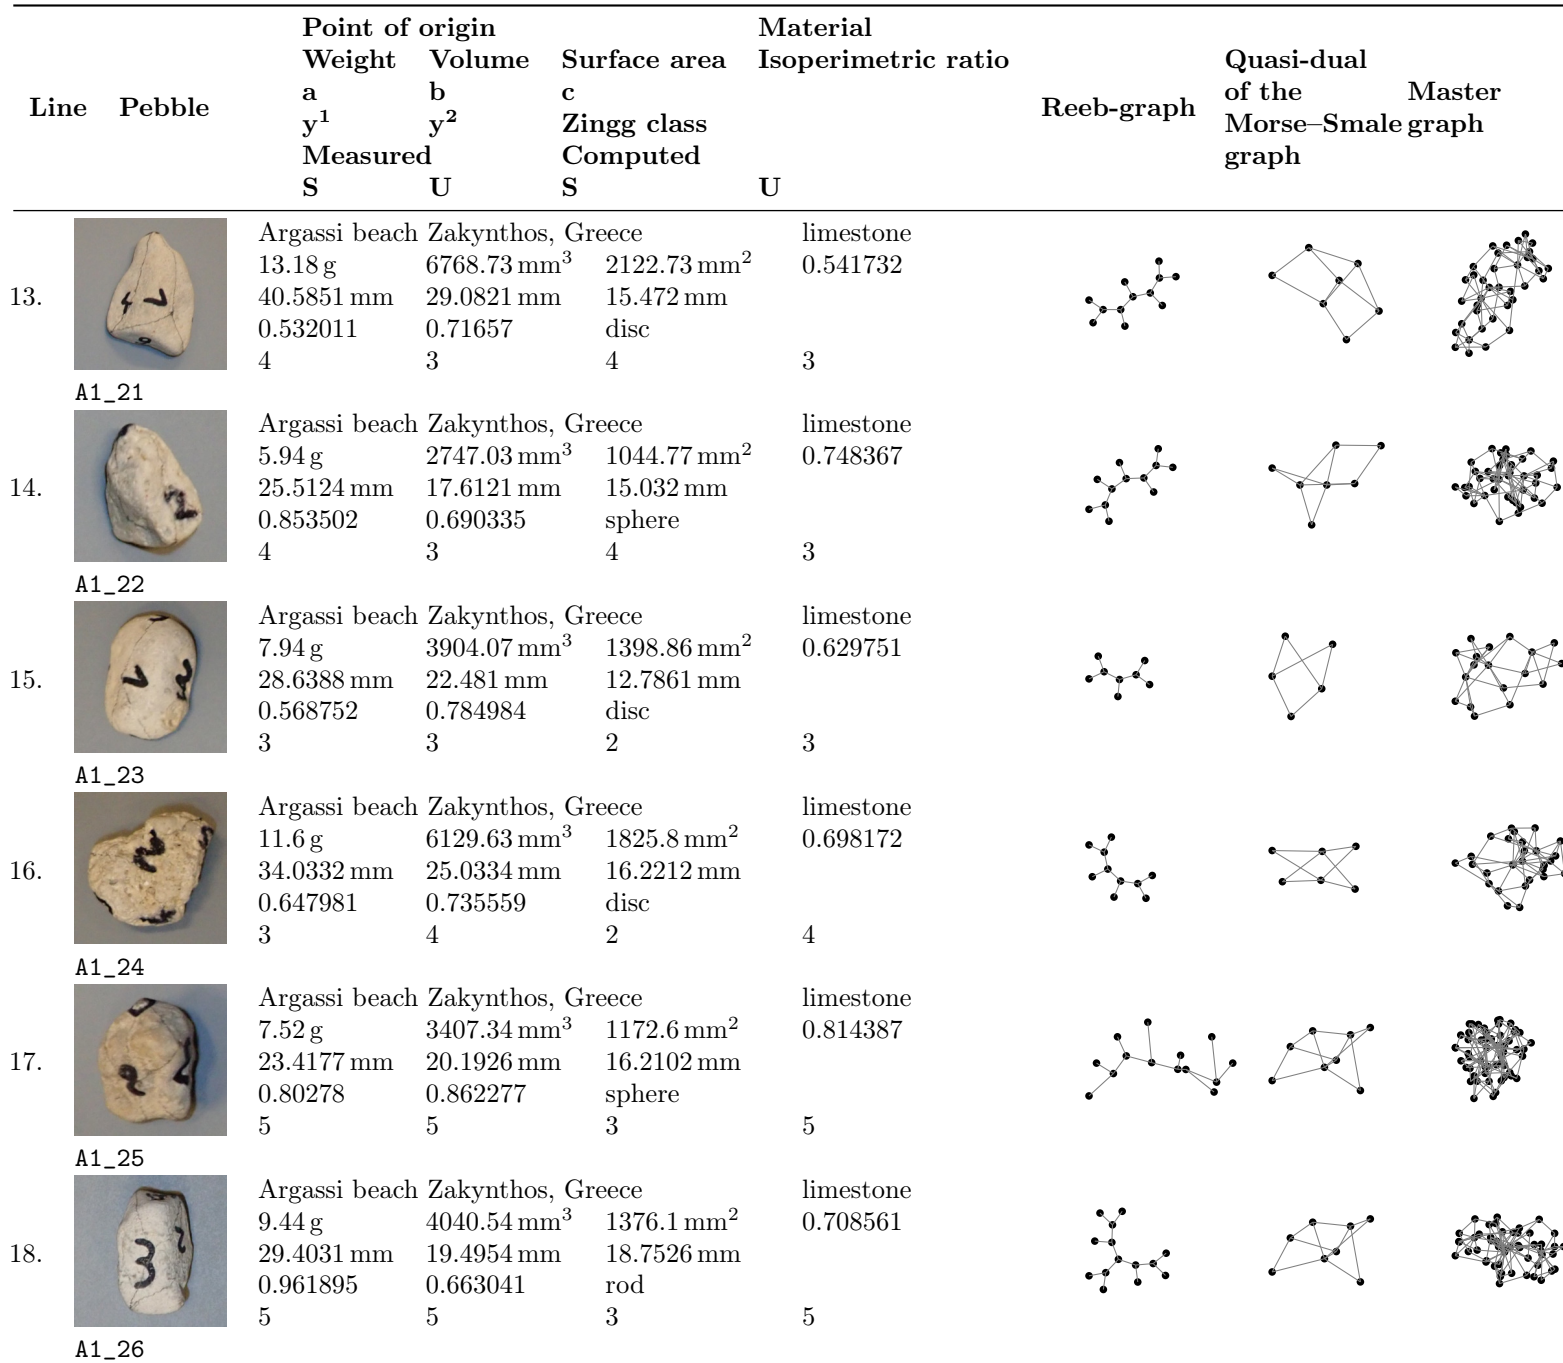   | 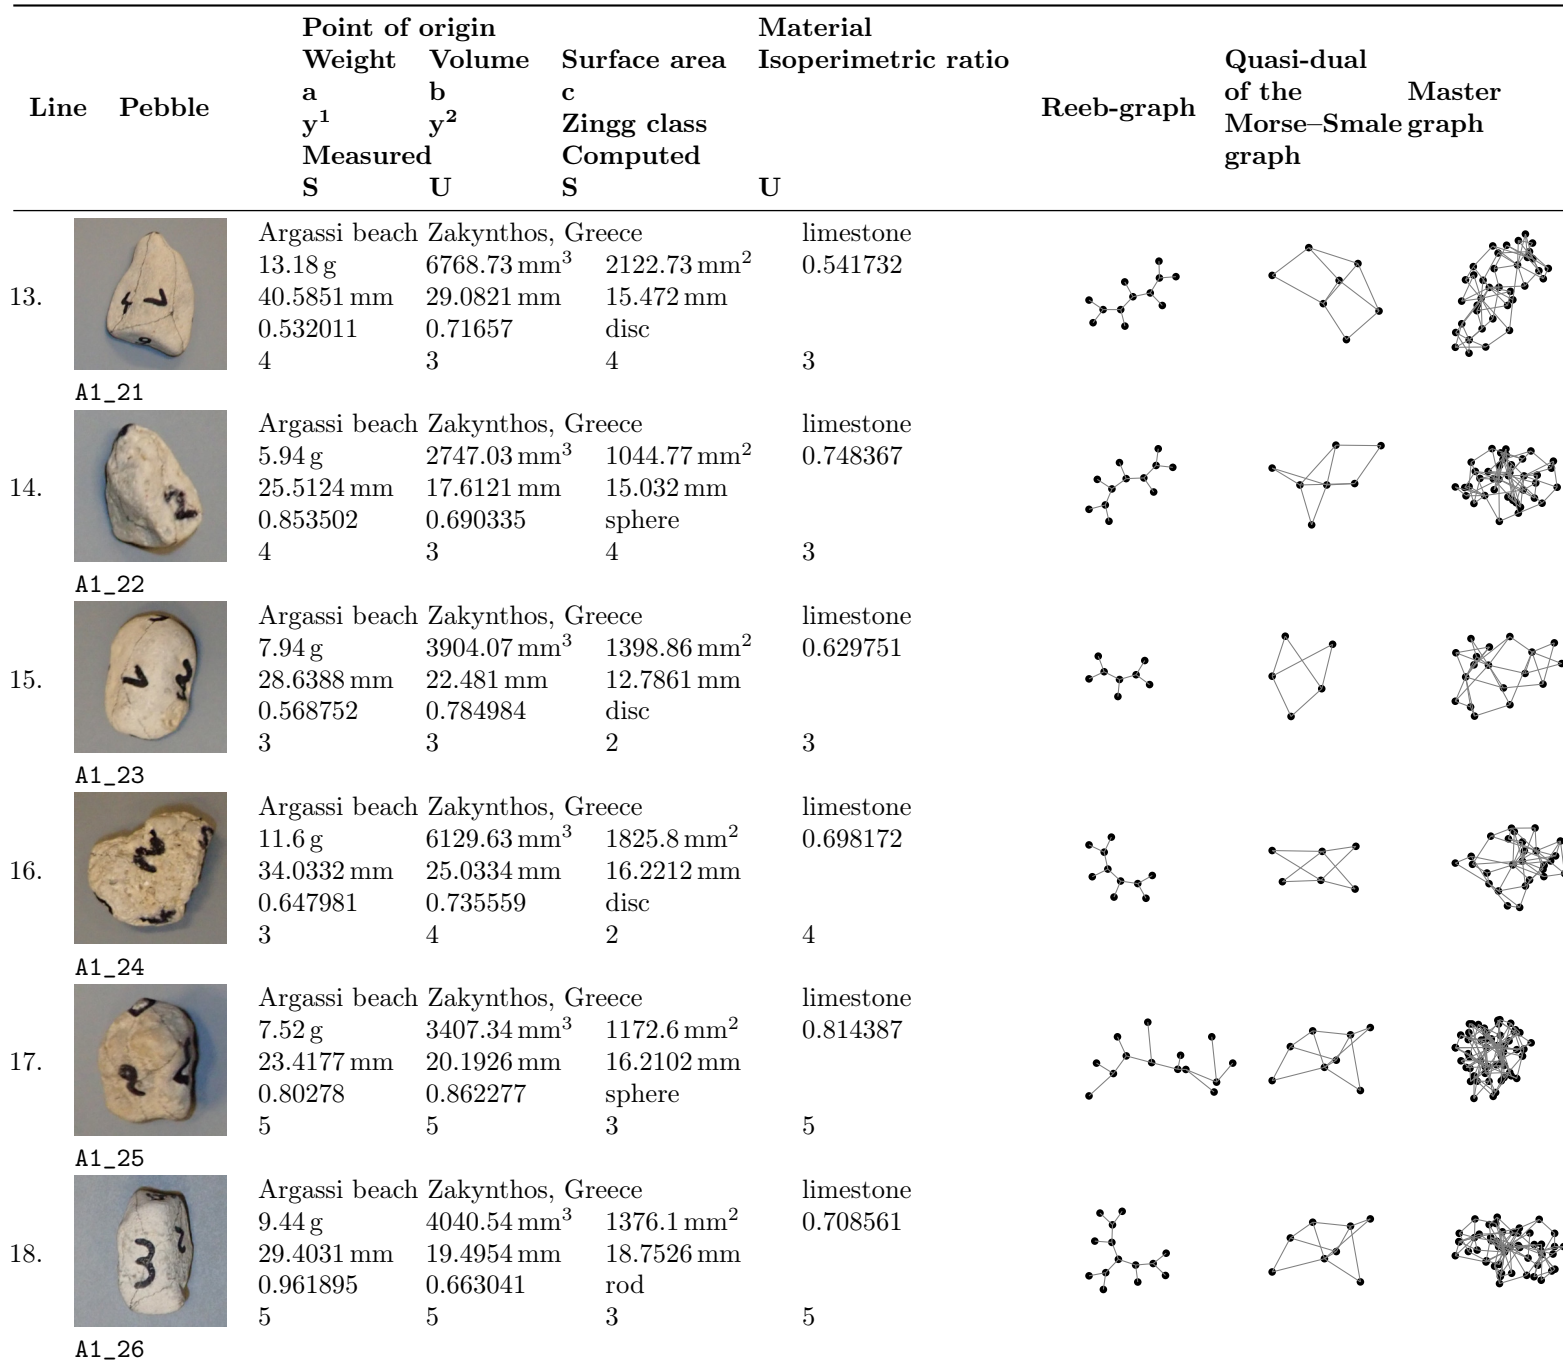   |
| A1_23 |                                                                                     |                                                         |                                                                             |                                                     |                                |                                                                                       |                                                                                       |                                                                                       |
| 16.   | 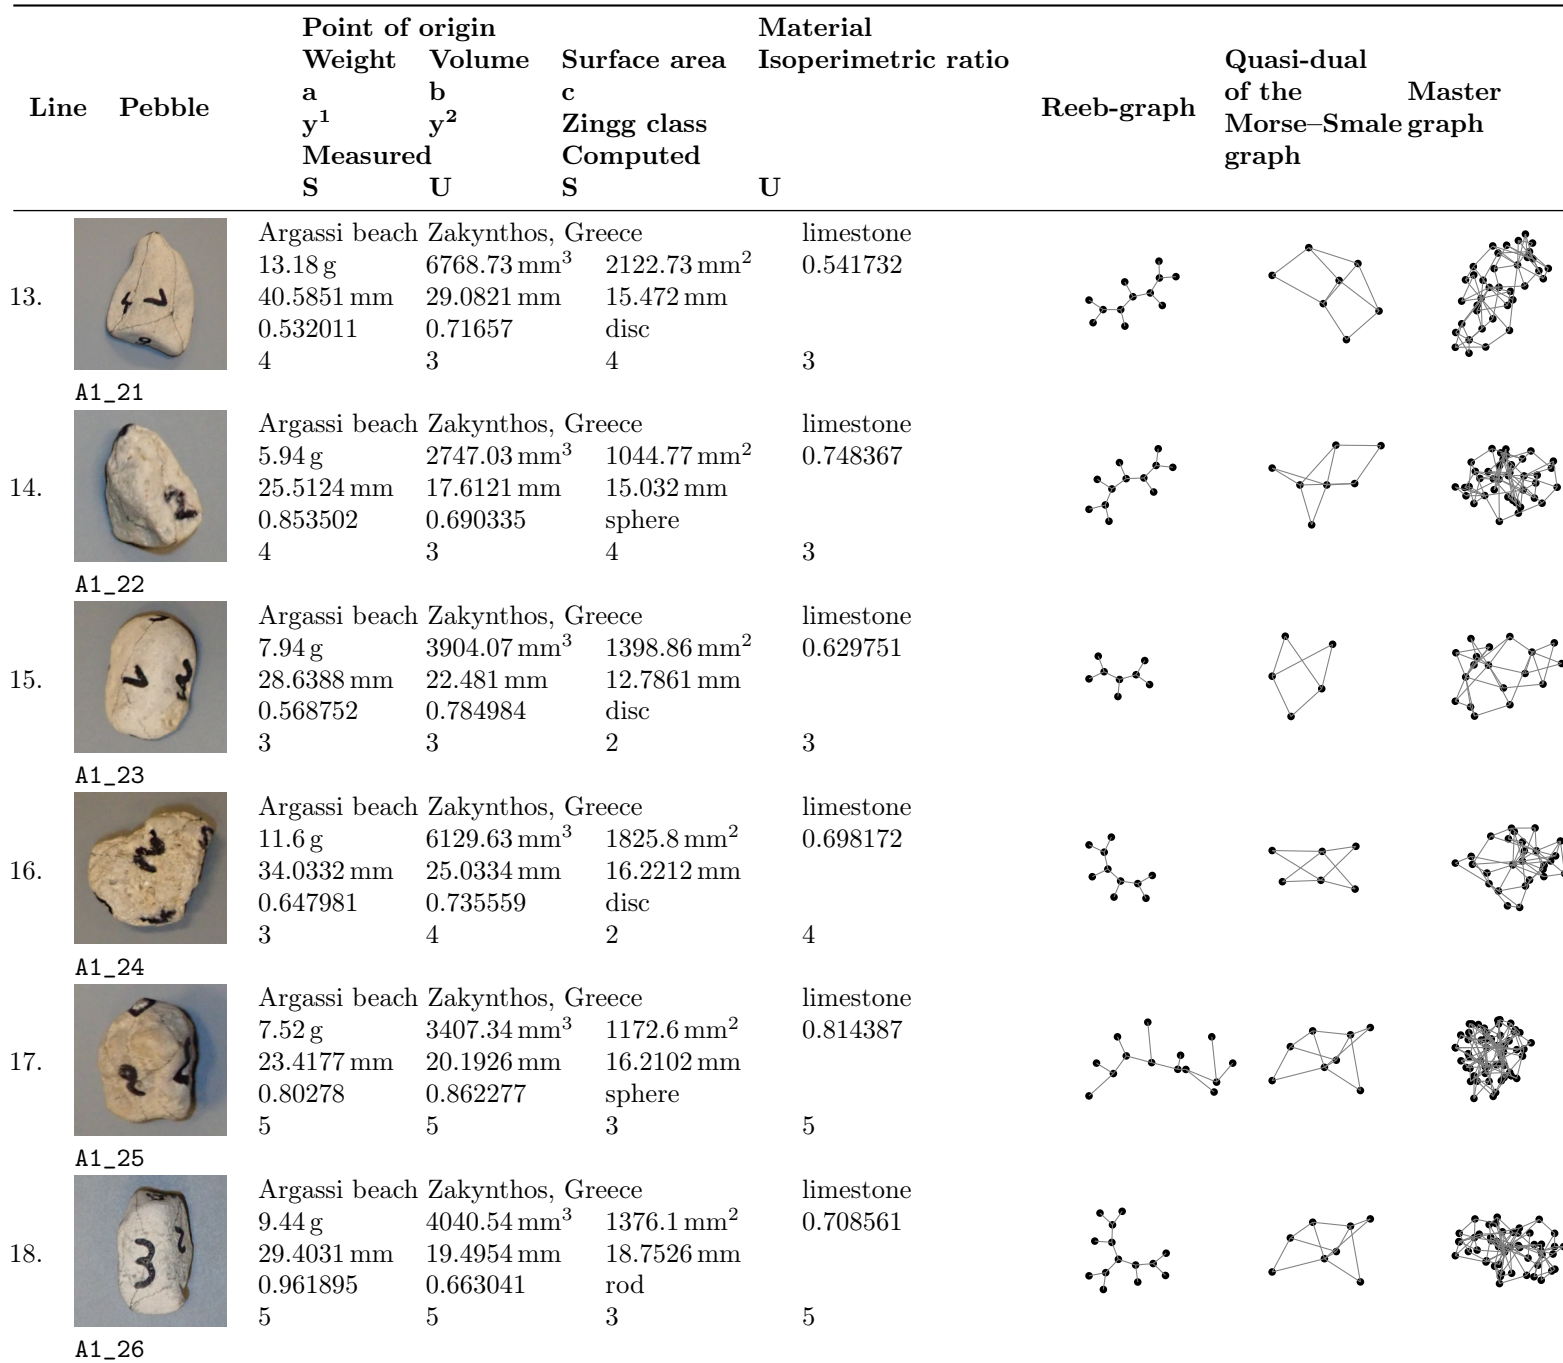  | Argassi beach<br>11.6 g<br>34.0332 mm<br>0.647981<br>3  | Zakynthos, Greece<br>6129.63 mm <sup>3</sup><br>25.0334 mm<br>0.735559<br>4 | 1825.8 mm <sup>2</sup><br>16.2212 mm<br>disc<br>2   | limestone<br>0.698172<br><br>4 | 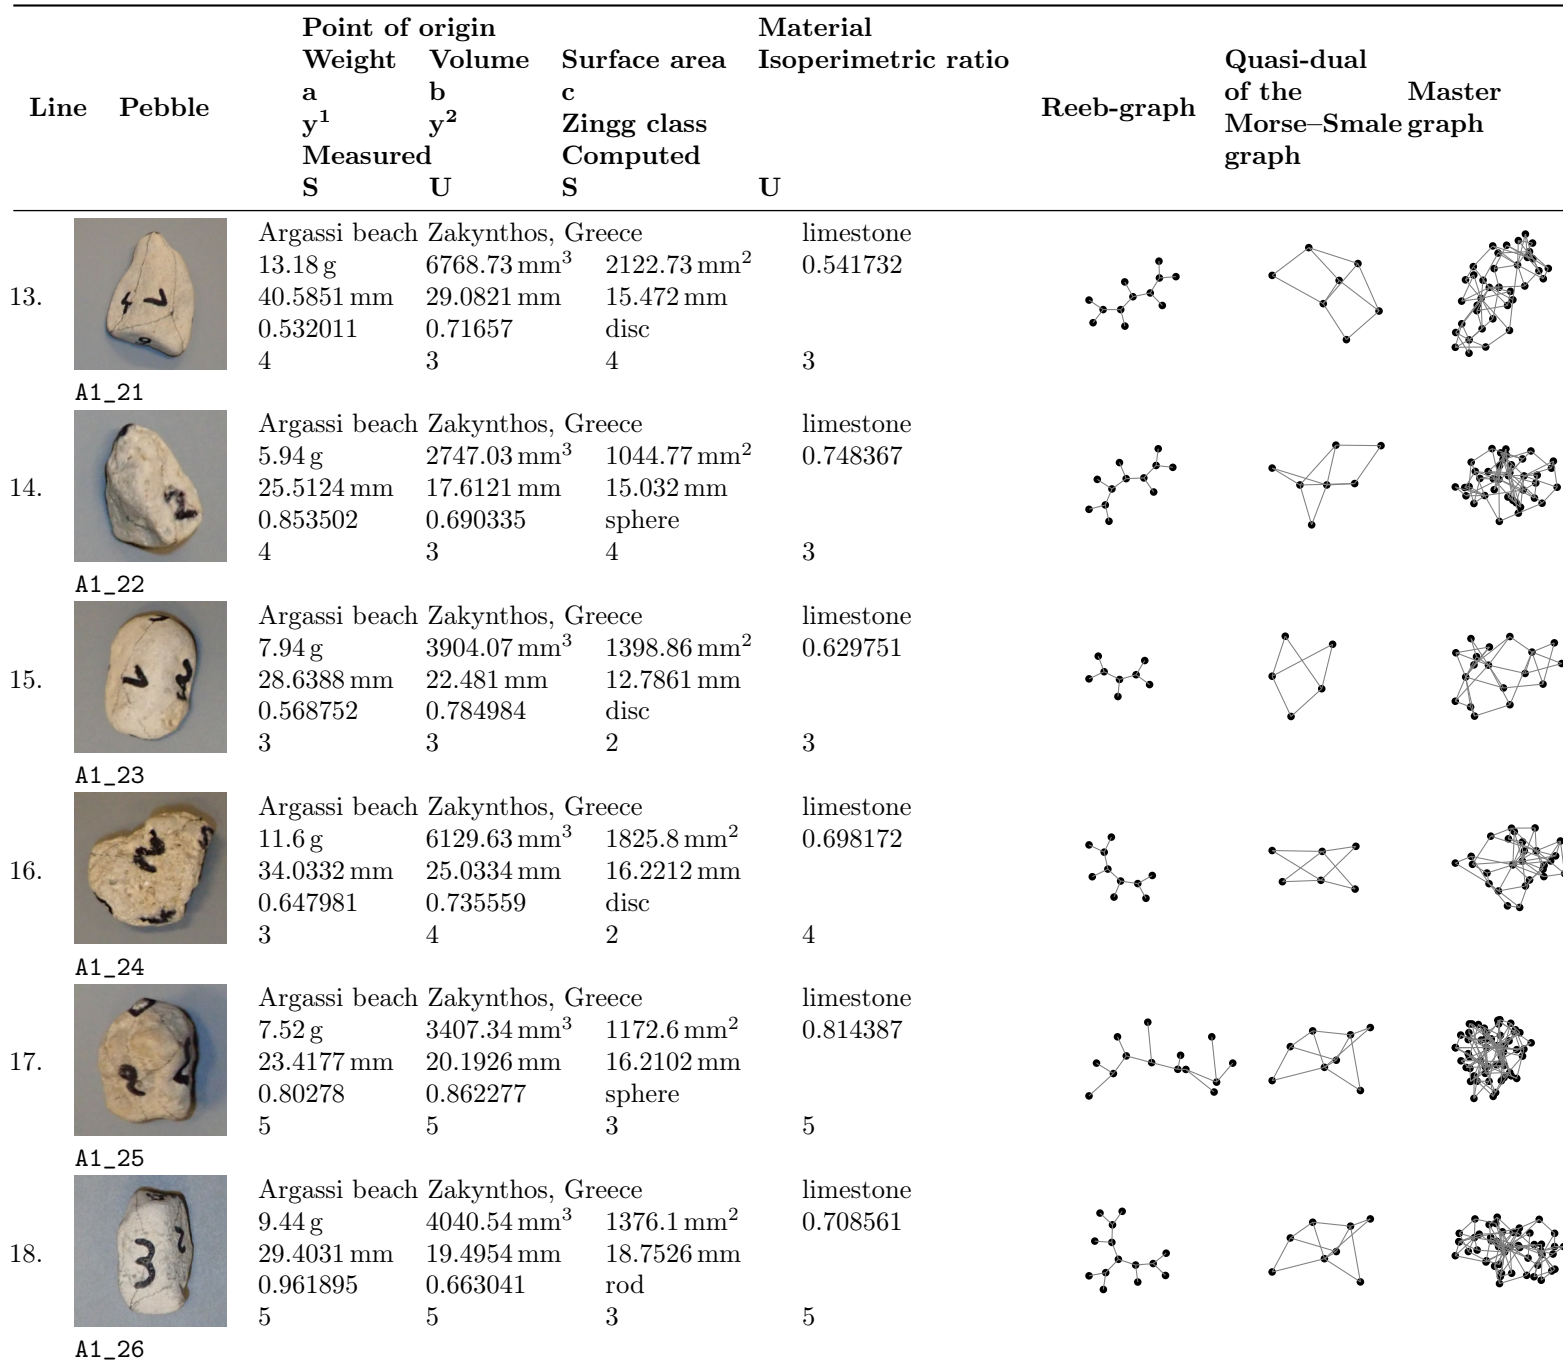  | 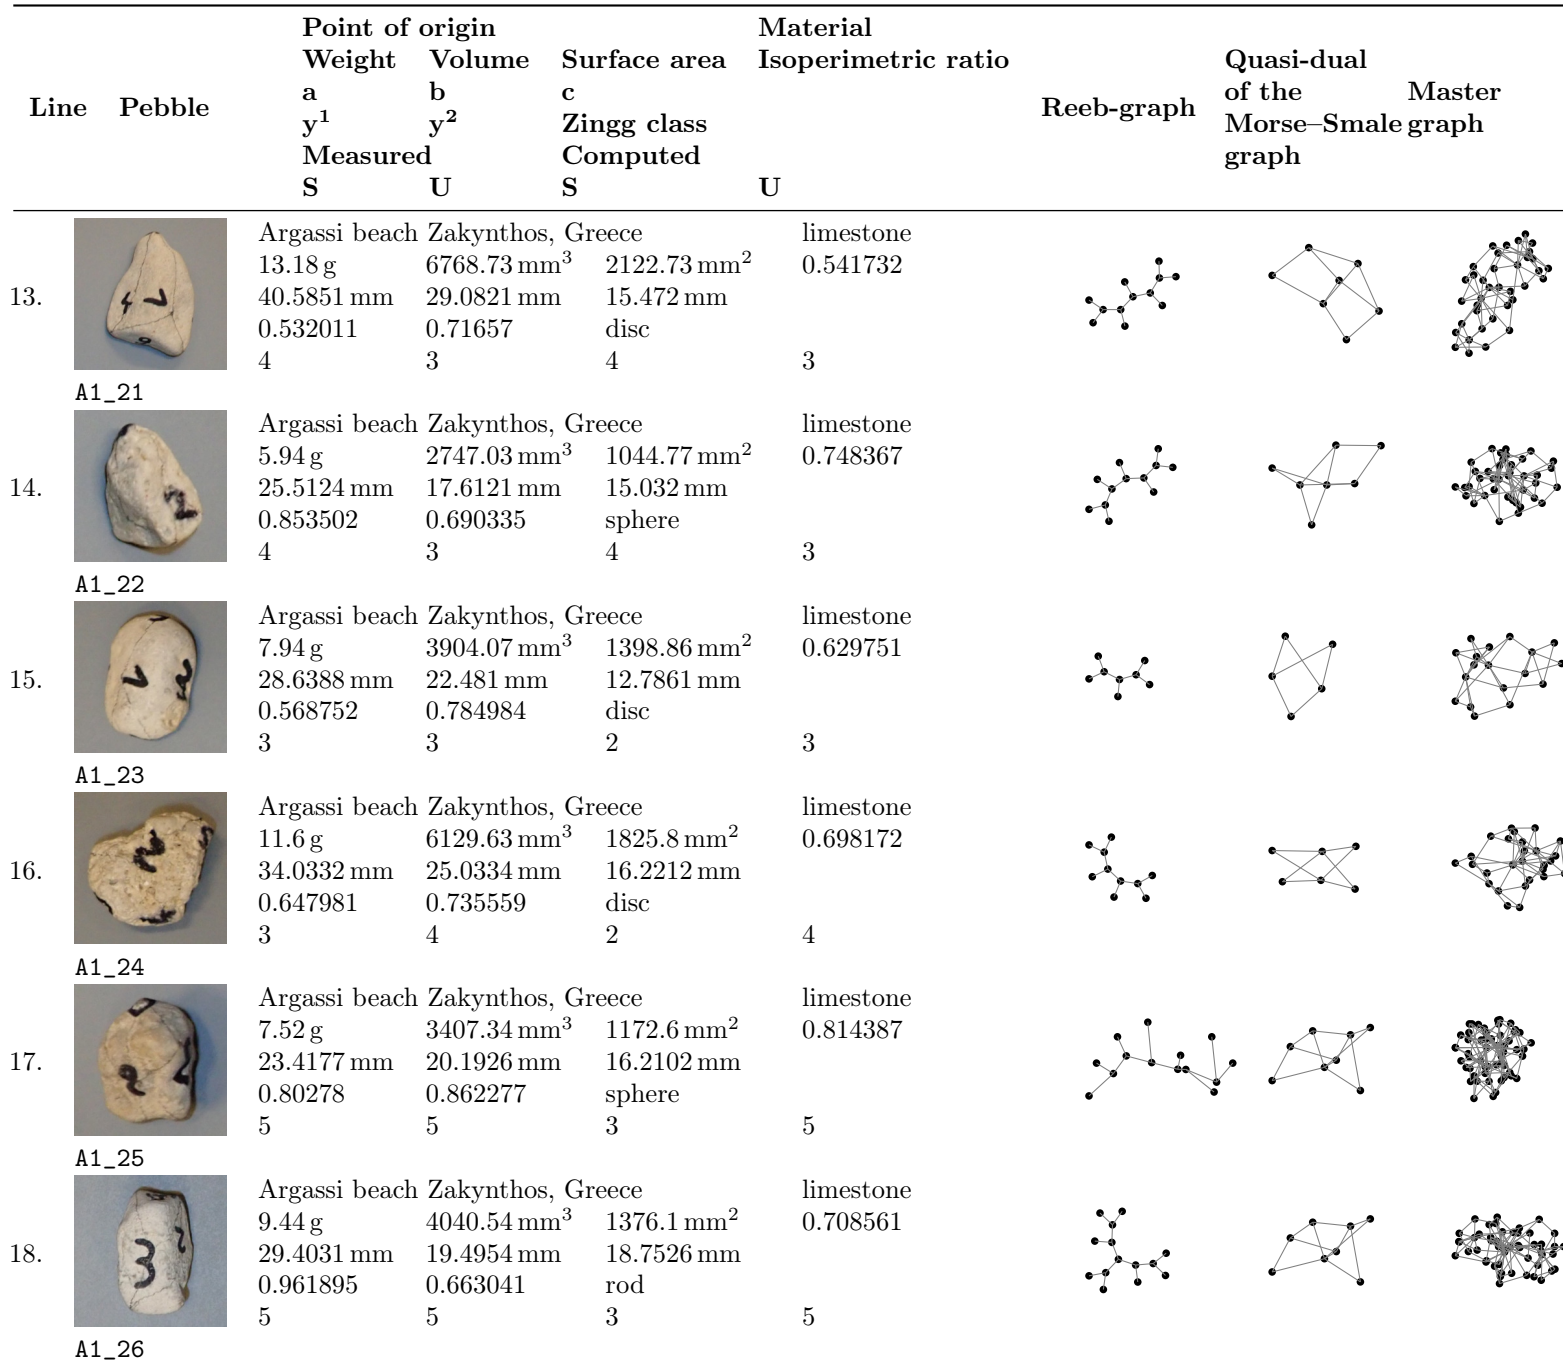  | 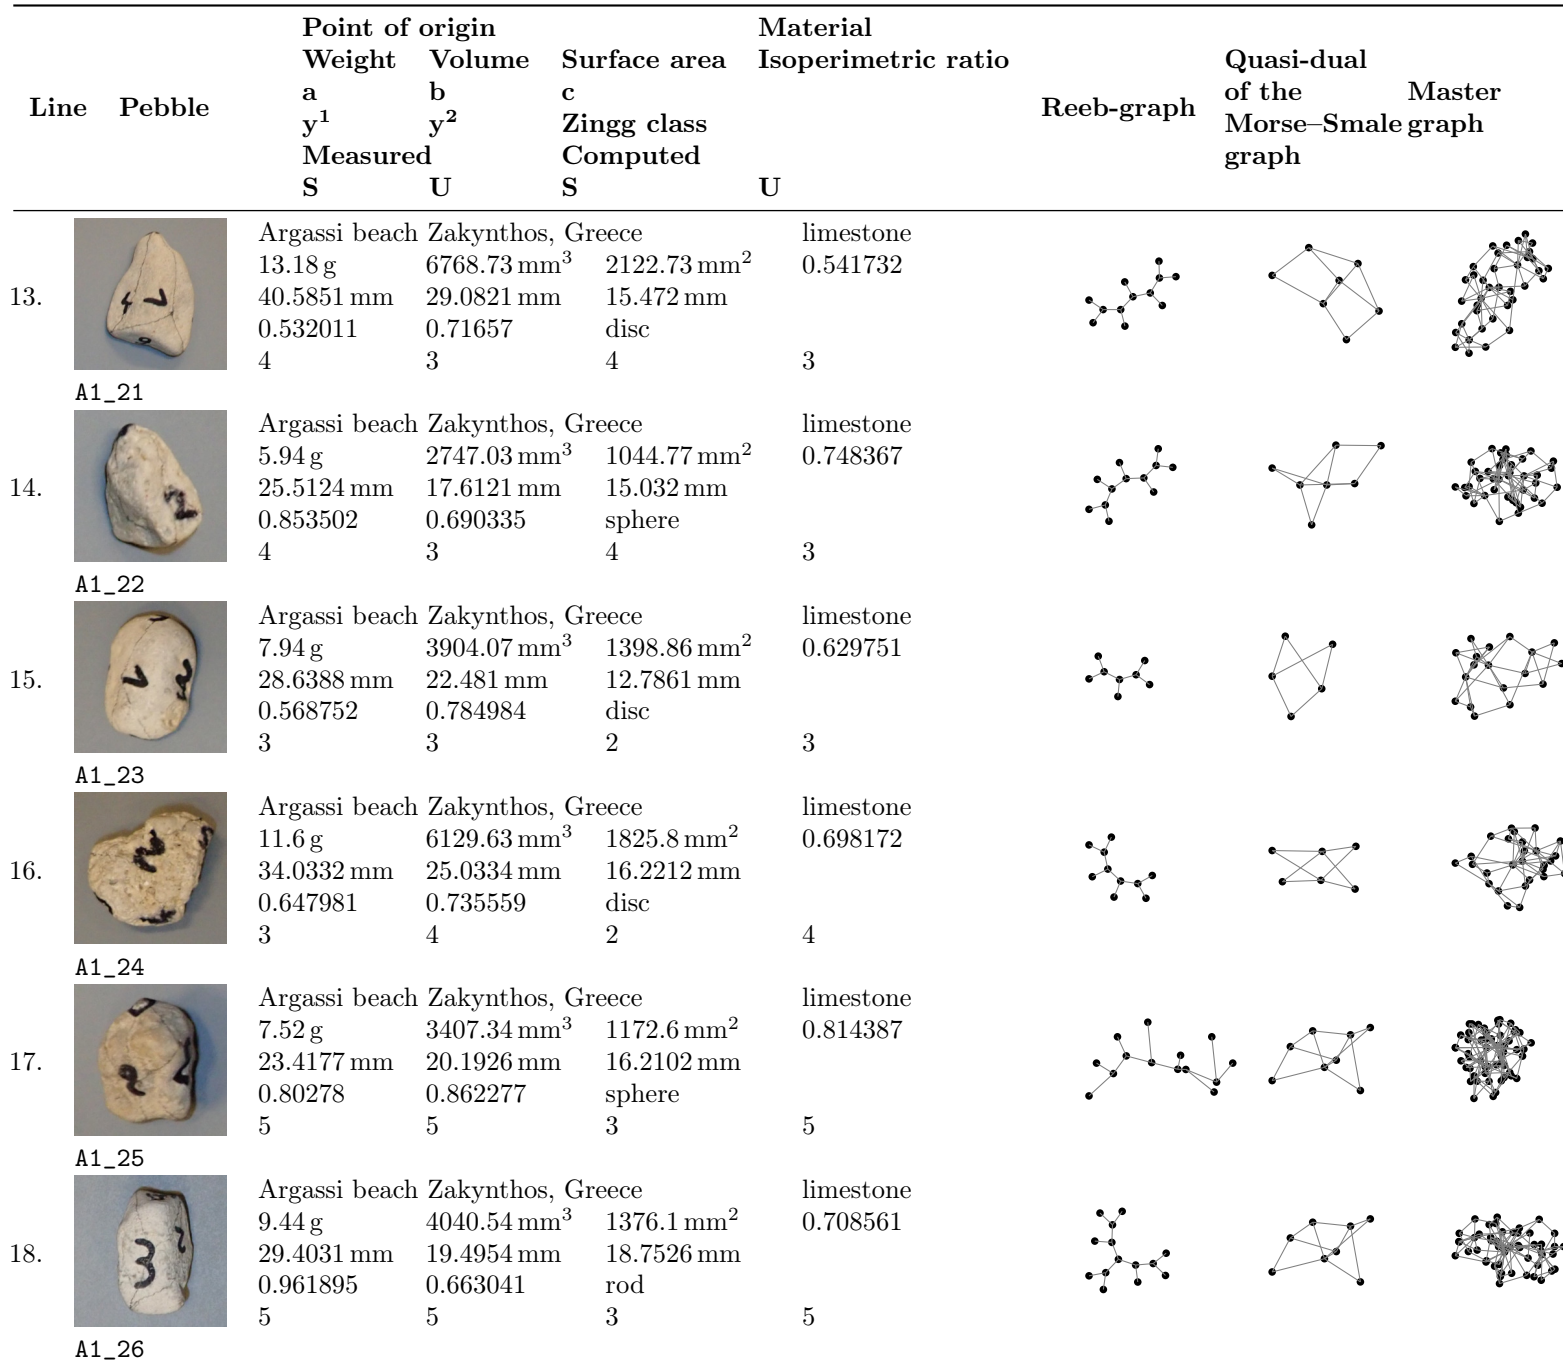  |
| A1_24 |                                                                                     |                                                         |                                                                             |                                                     |                                |                                                                                       |                                                                                       |                                                                                       |
| 17.   | 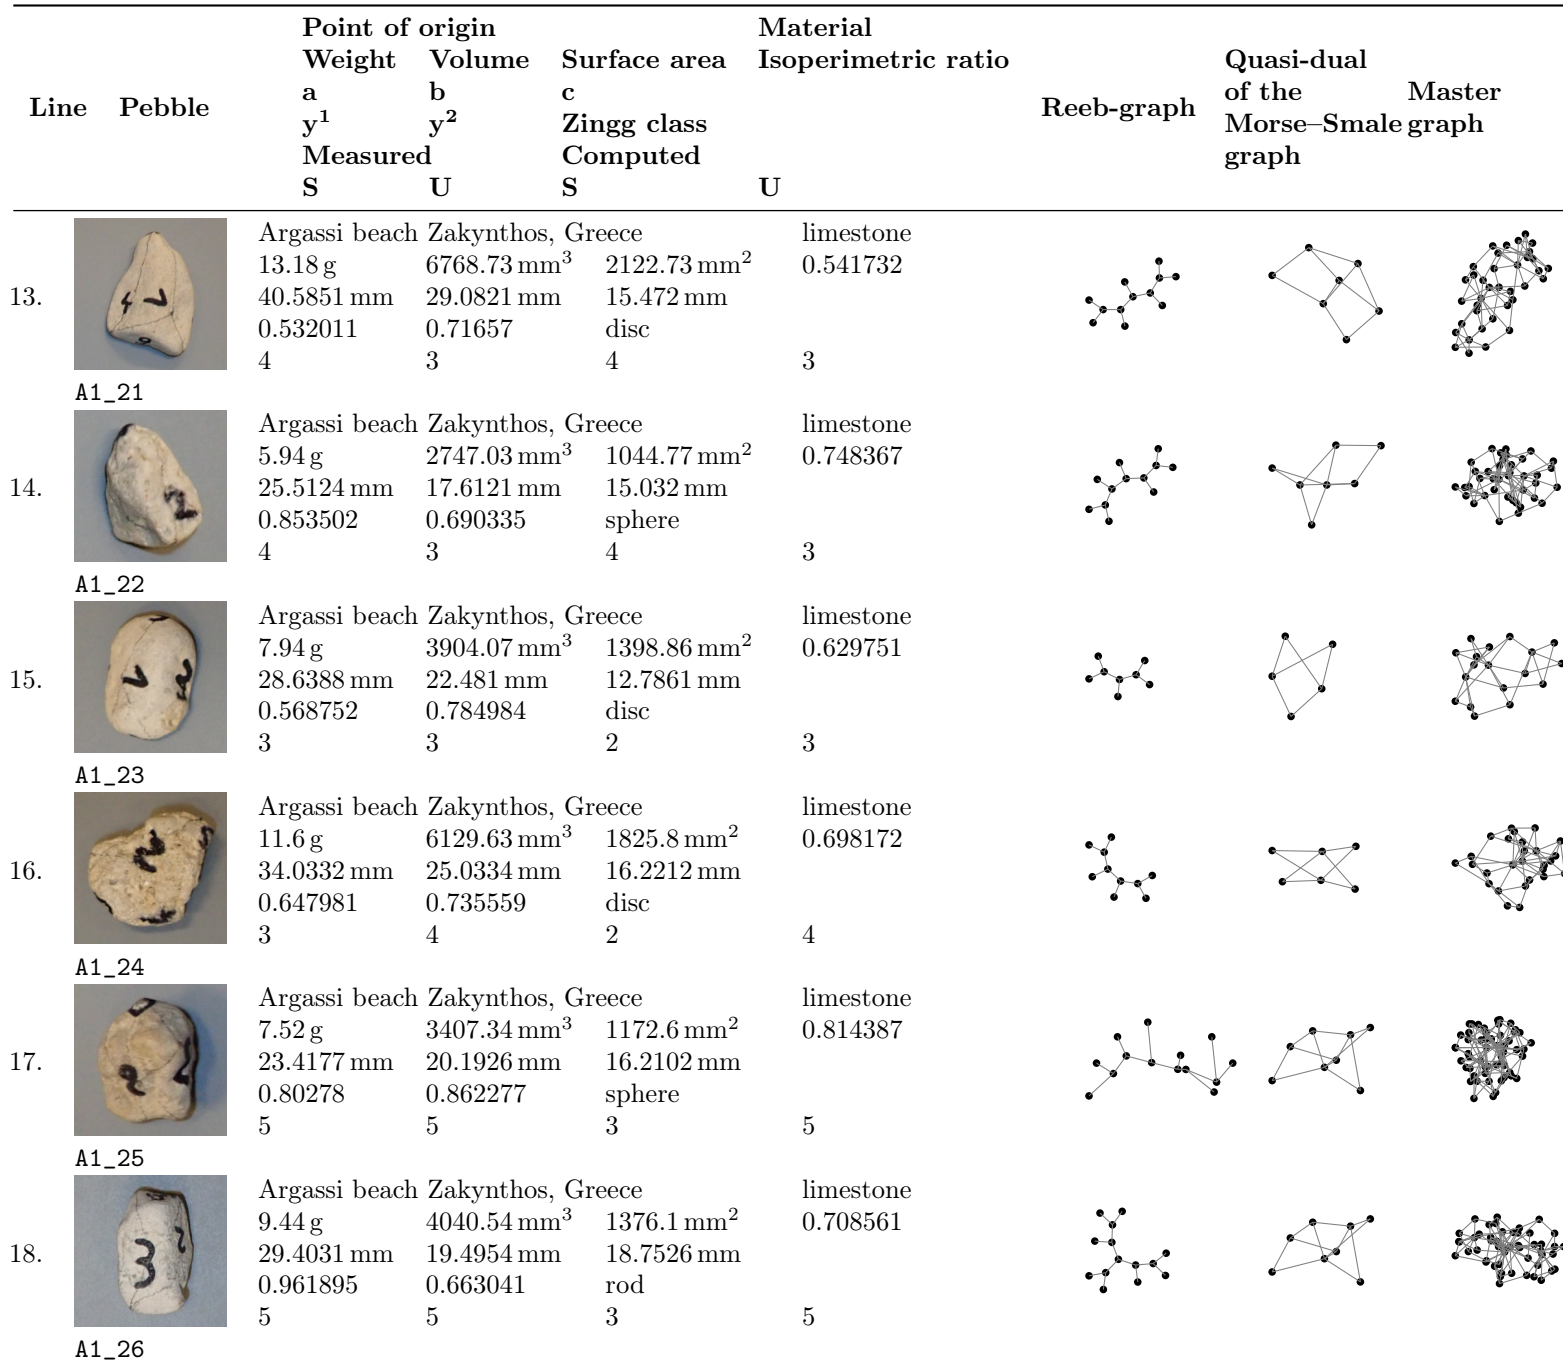 | Argassi beach<br>7.52 g<br>23.4177 mm<br>0.80278<br>5   | Zakynthos, Greece<br>3407.34 mm <sup>3</sup><br>20.1926 mm<br>0.862277<br>5 | 1172.6 mm <sup>2</sup><br>16.2102 mm<br>sphere<br>3 | limestone<br>0.814387<br><br>5 | 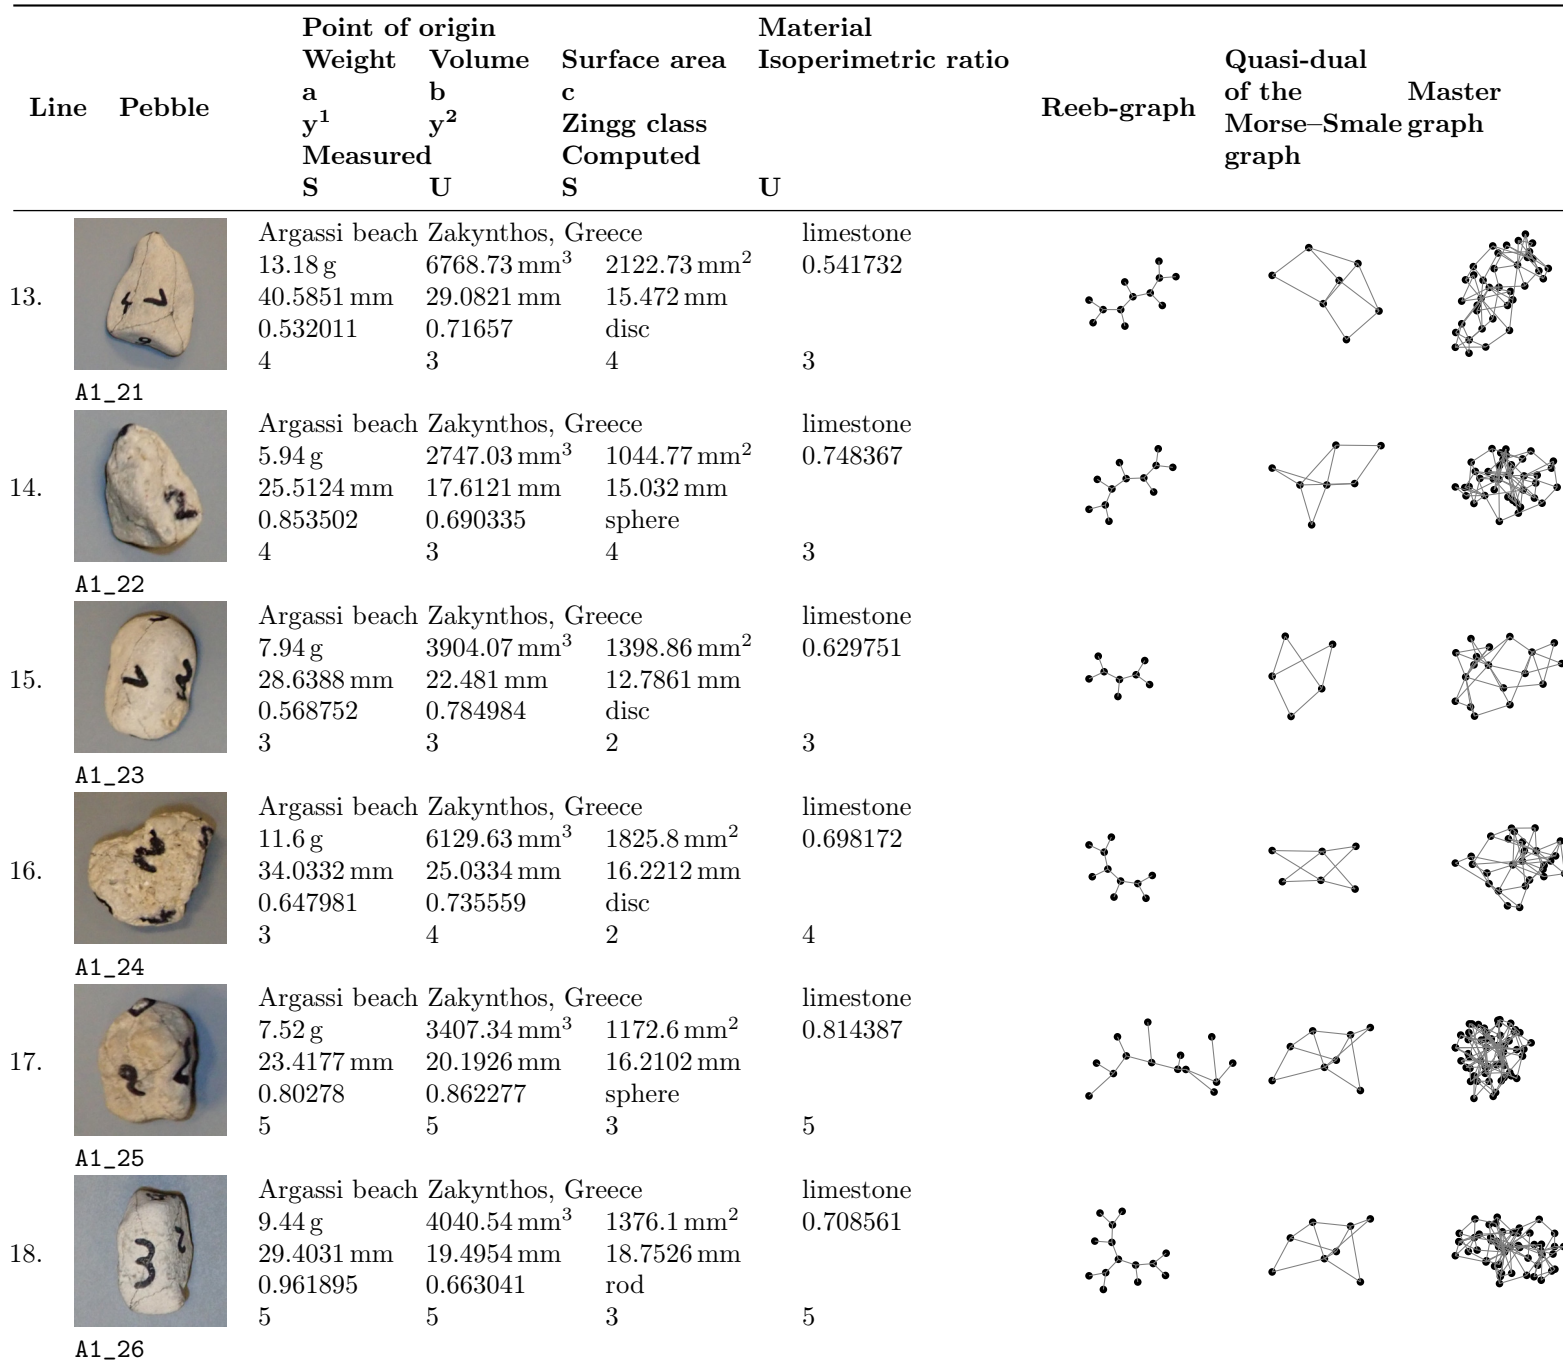 | 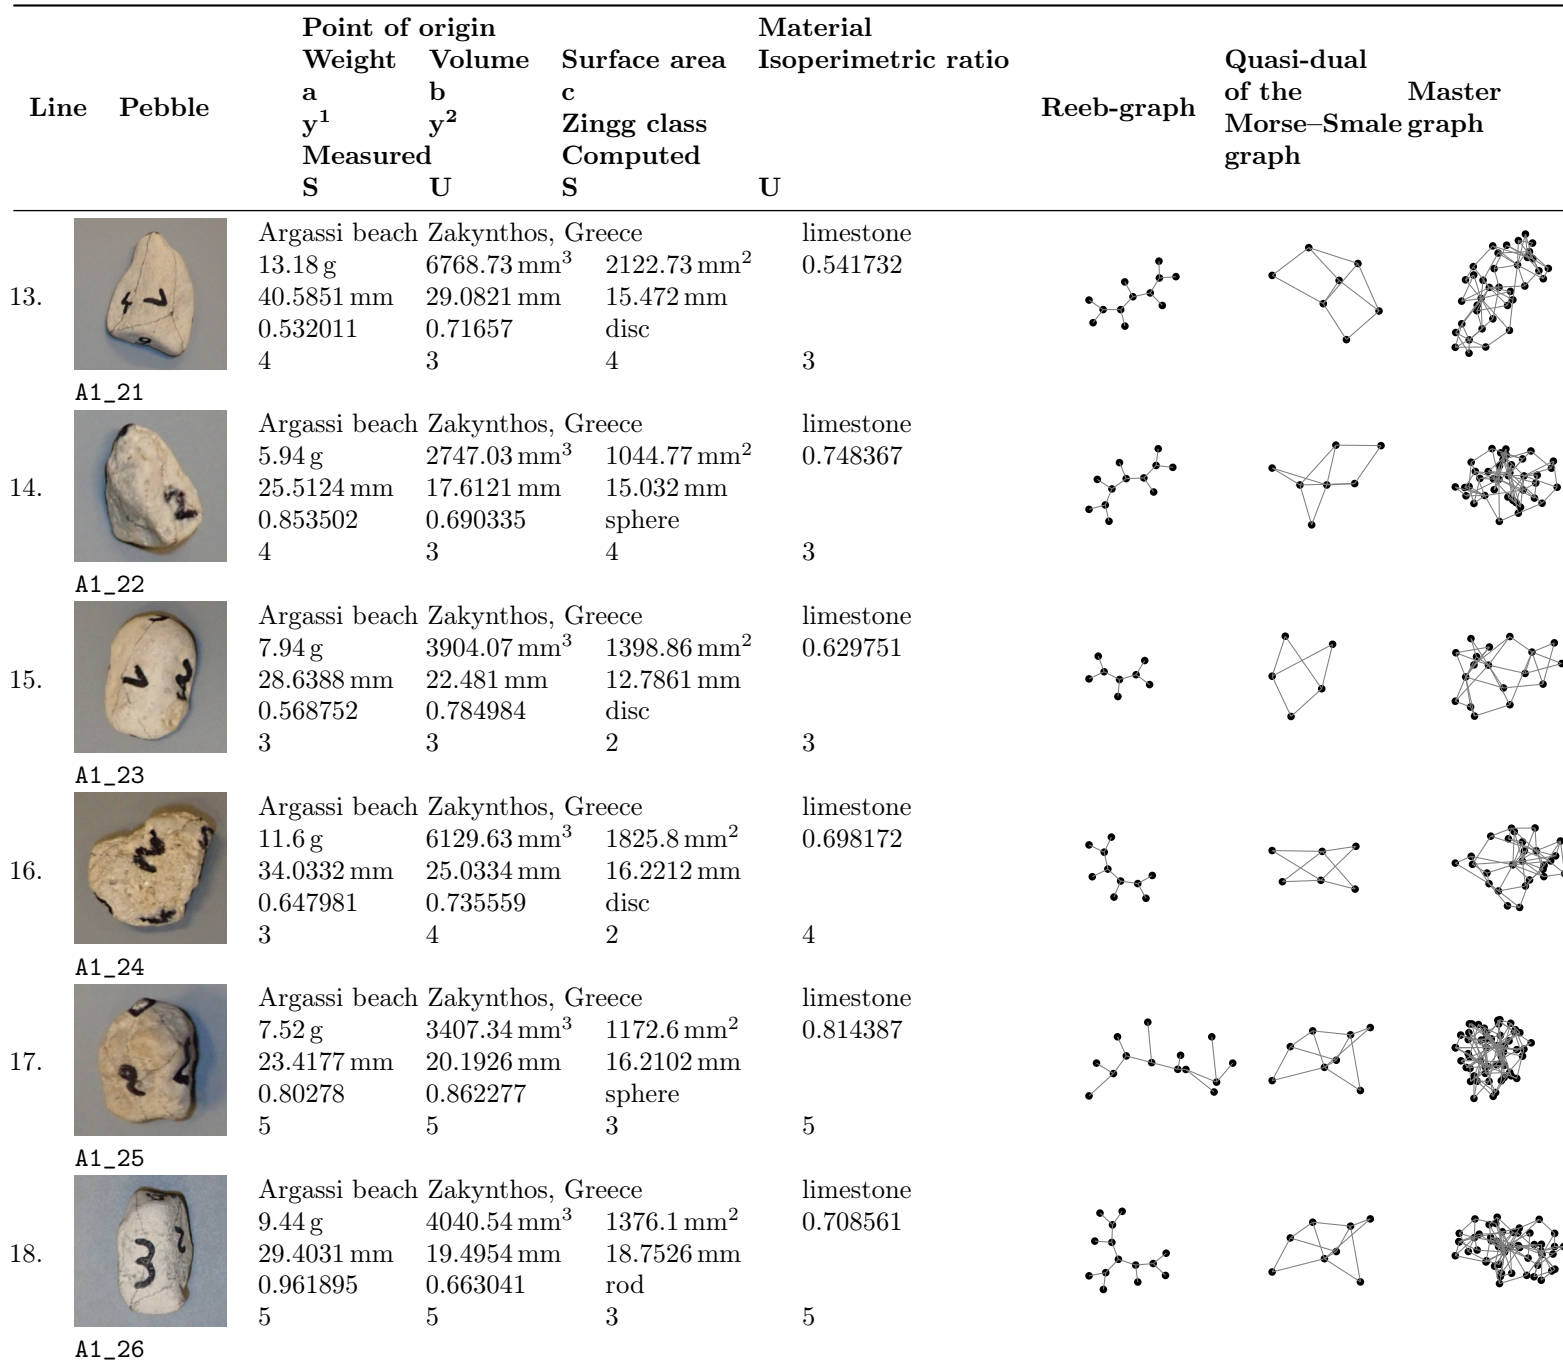 | 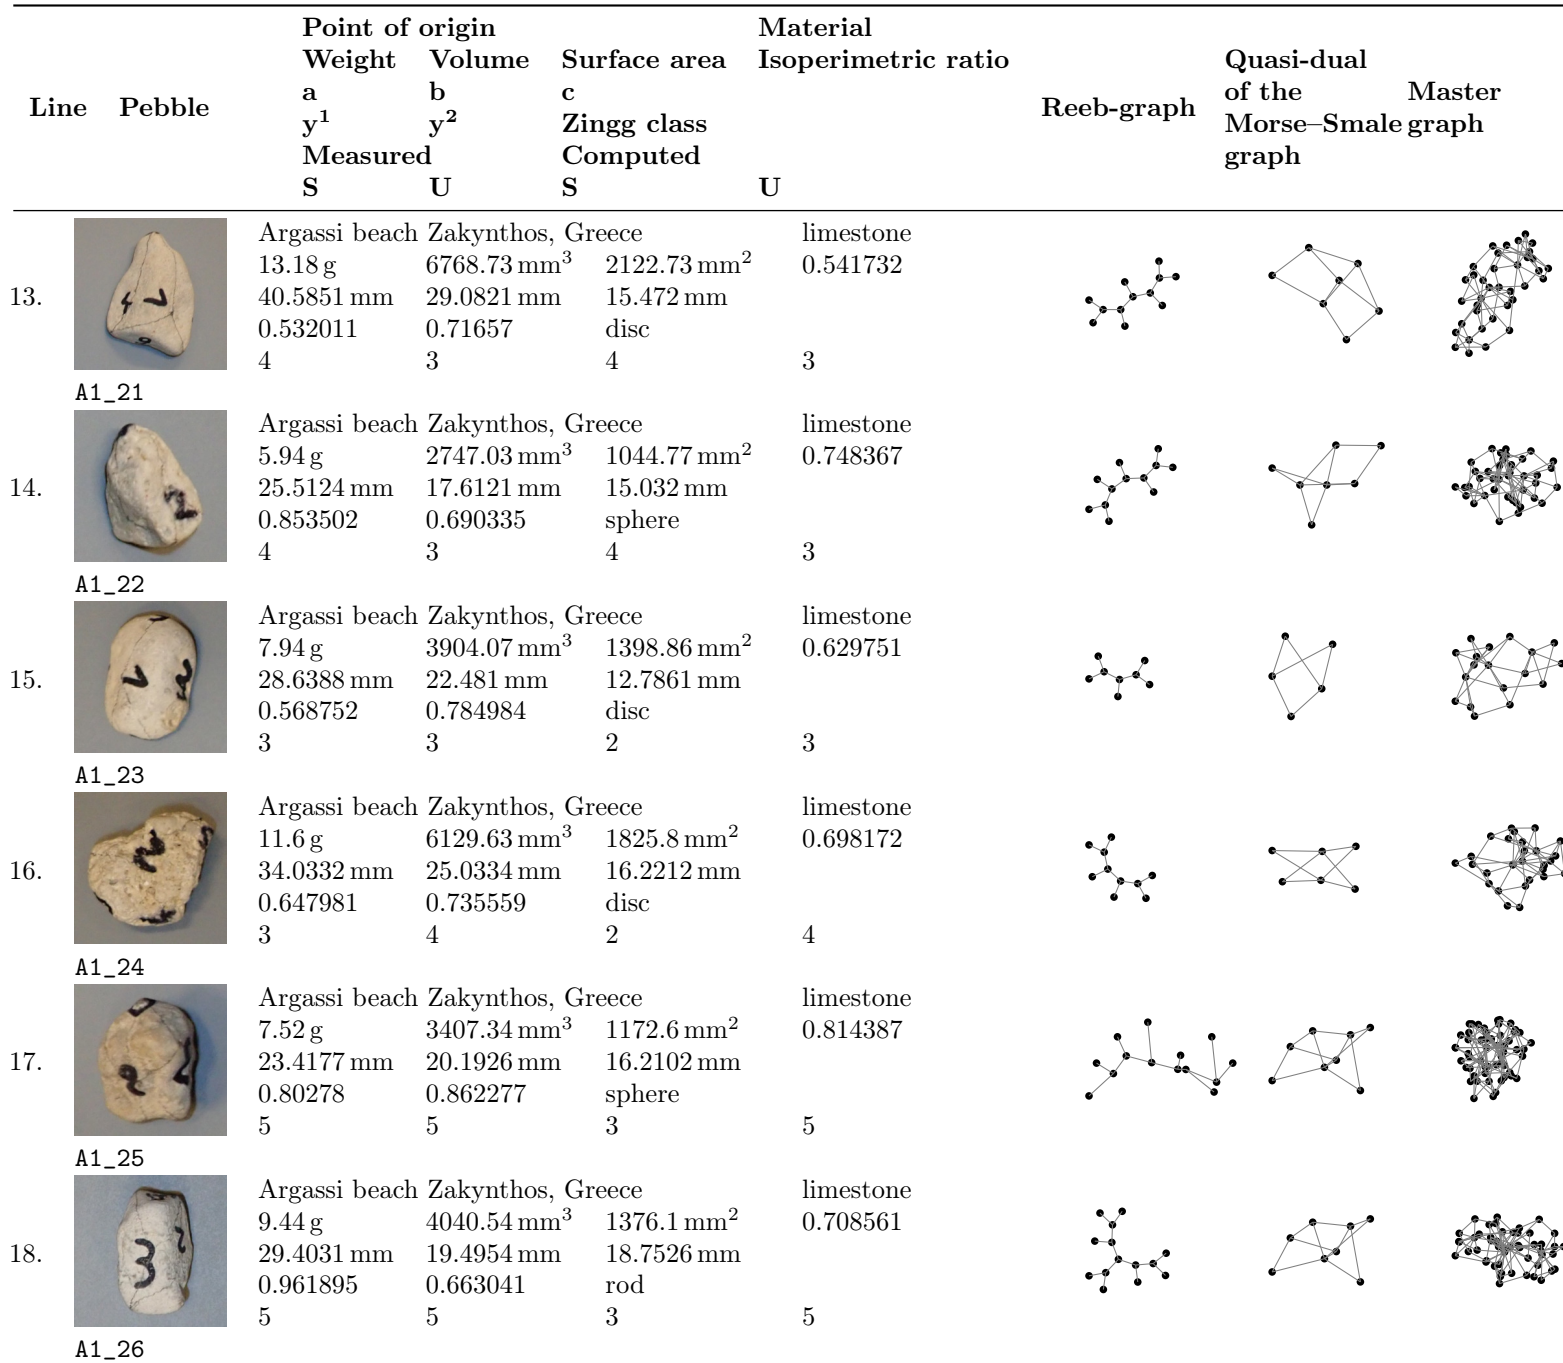 |
| A1_25 |                                                                                     |                                                         |                                                                             |                                                     |                                |                                                                                       |                                                                                       |                                                                                       |
| 18.   | 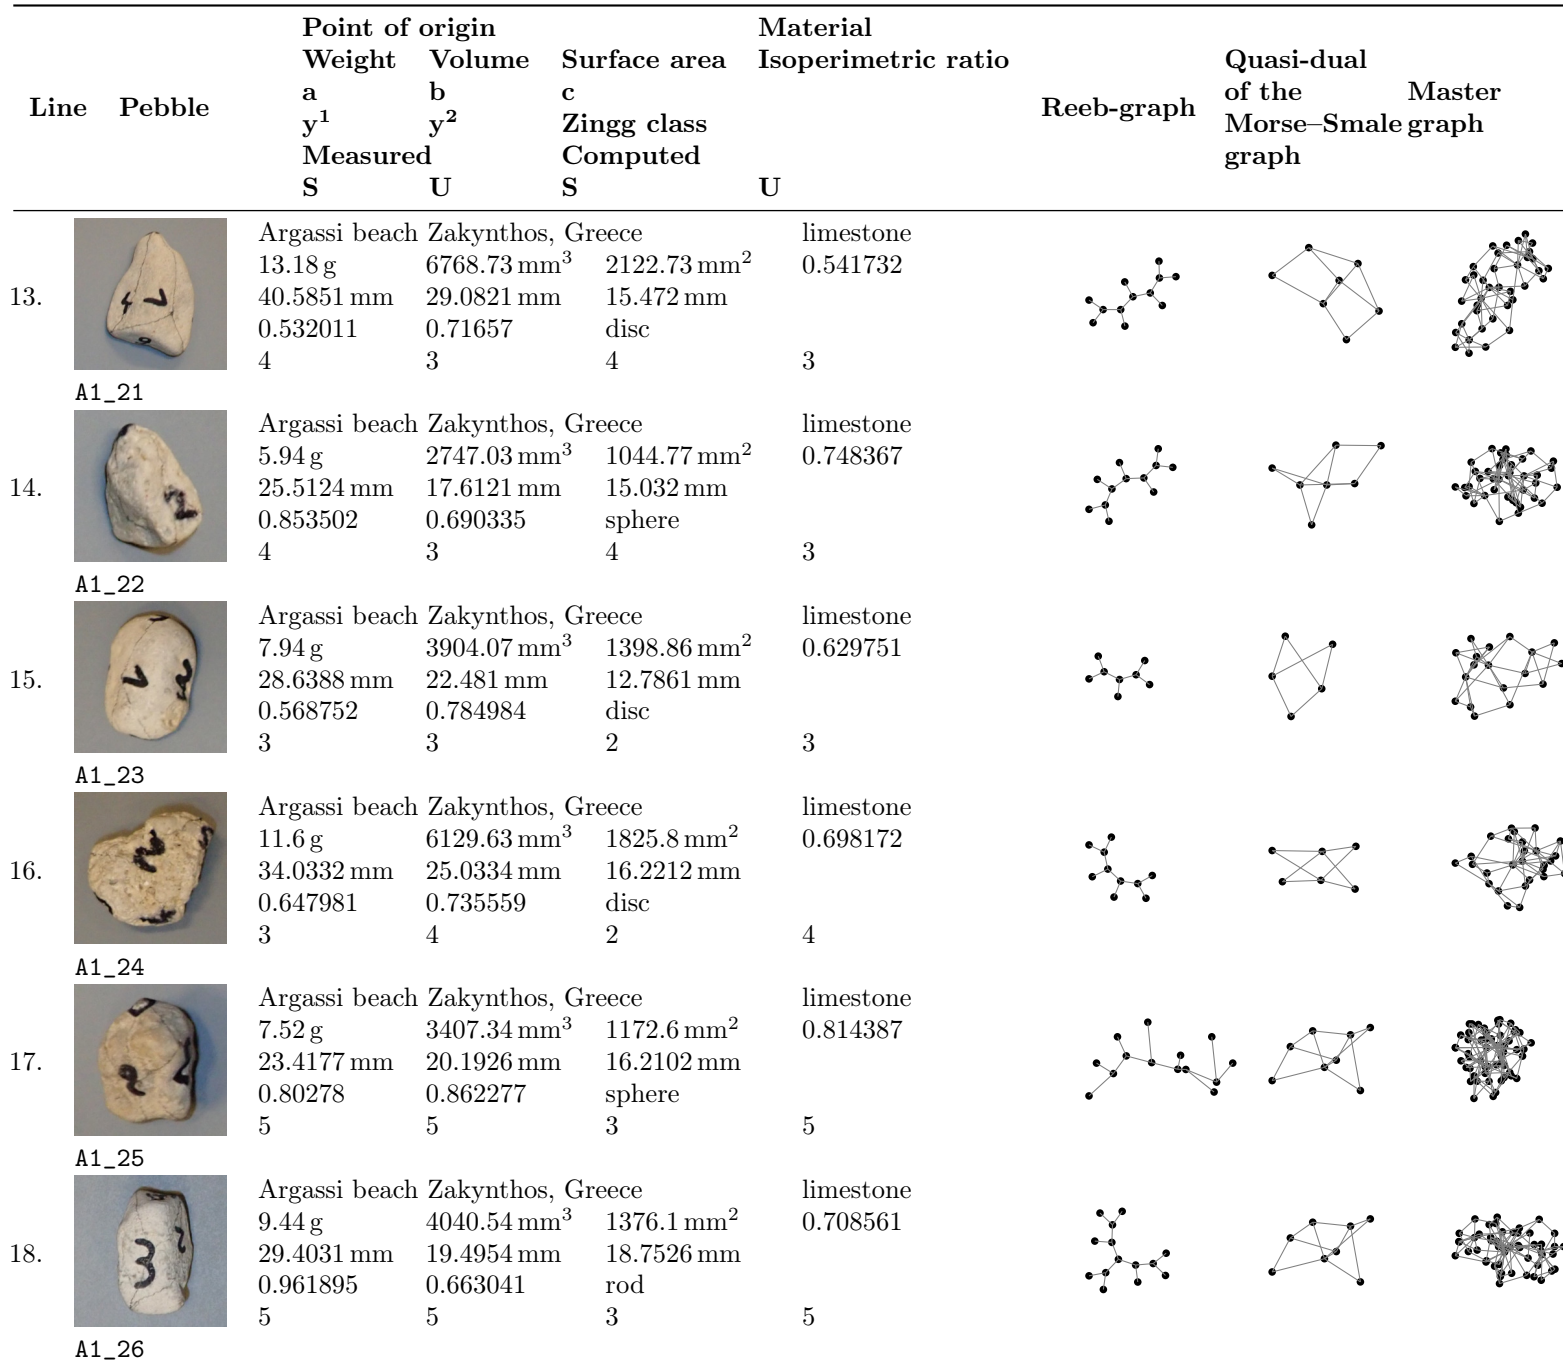 | Argassi beach<br>9.44 g<br>29.4031 mm<br>0.961895<br>5  | Zakynthos, Greece<br>4040.54 mm <sup>3</sup><br>19.4954 mm<br>0.663041<br>5 | 1376.1 mm <sup>2</sup><br>18.7526 mm<br>rod<br>3    | limestone<br>0.708561<br><br>5 | 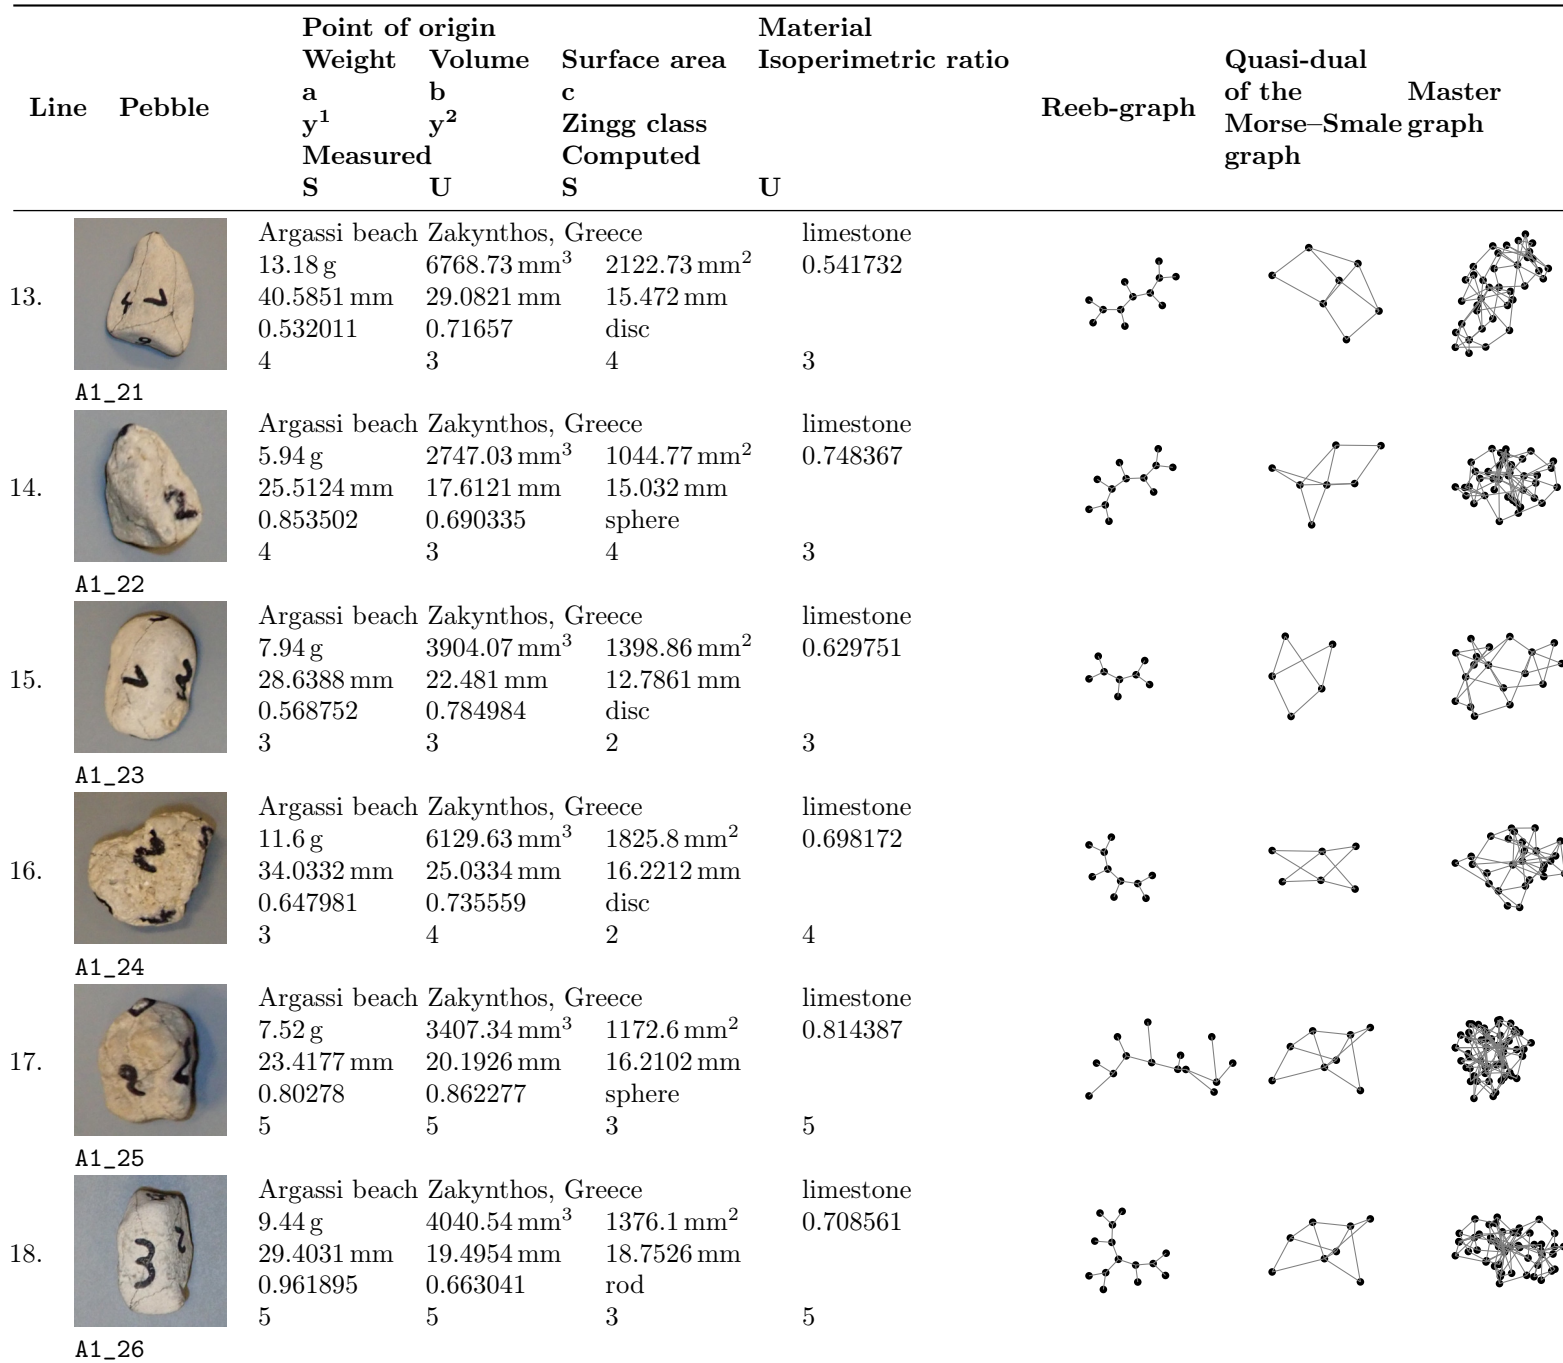 | 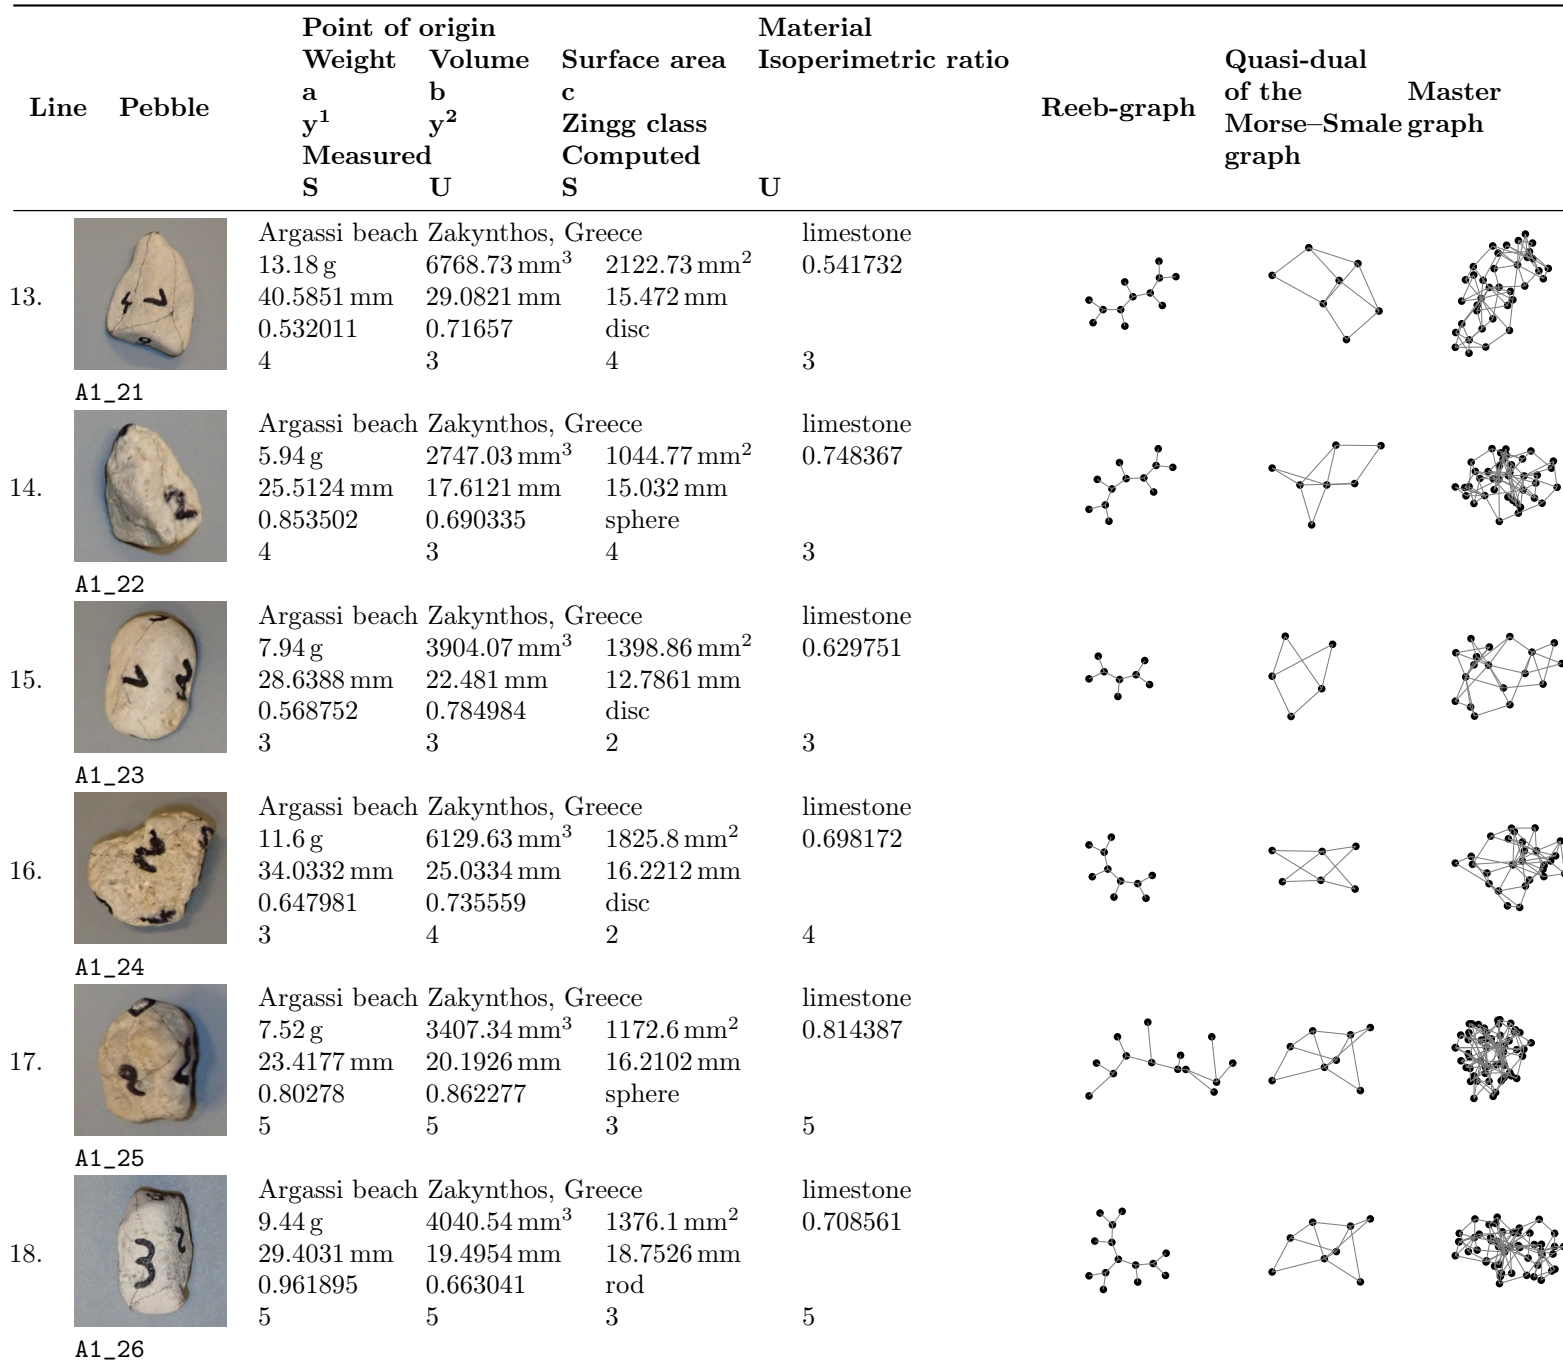 | 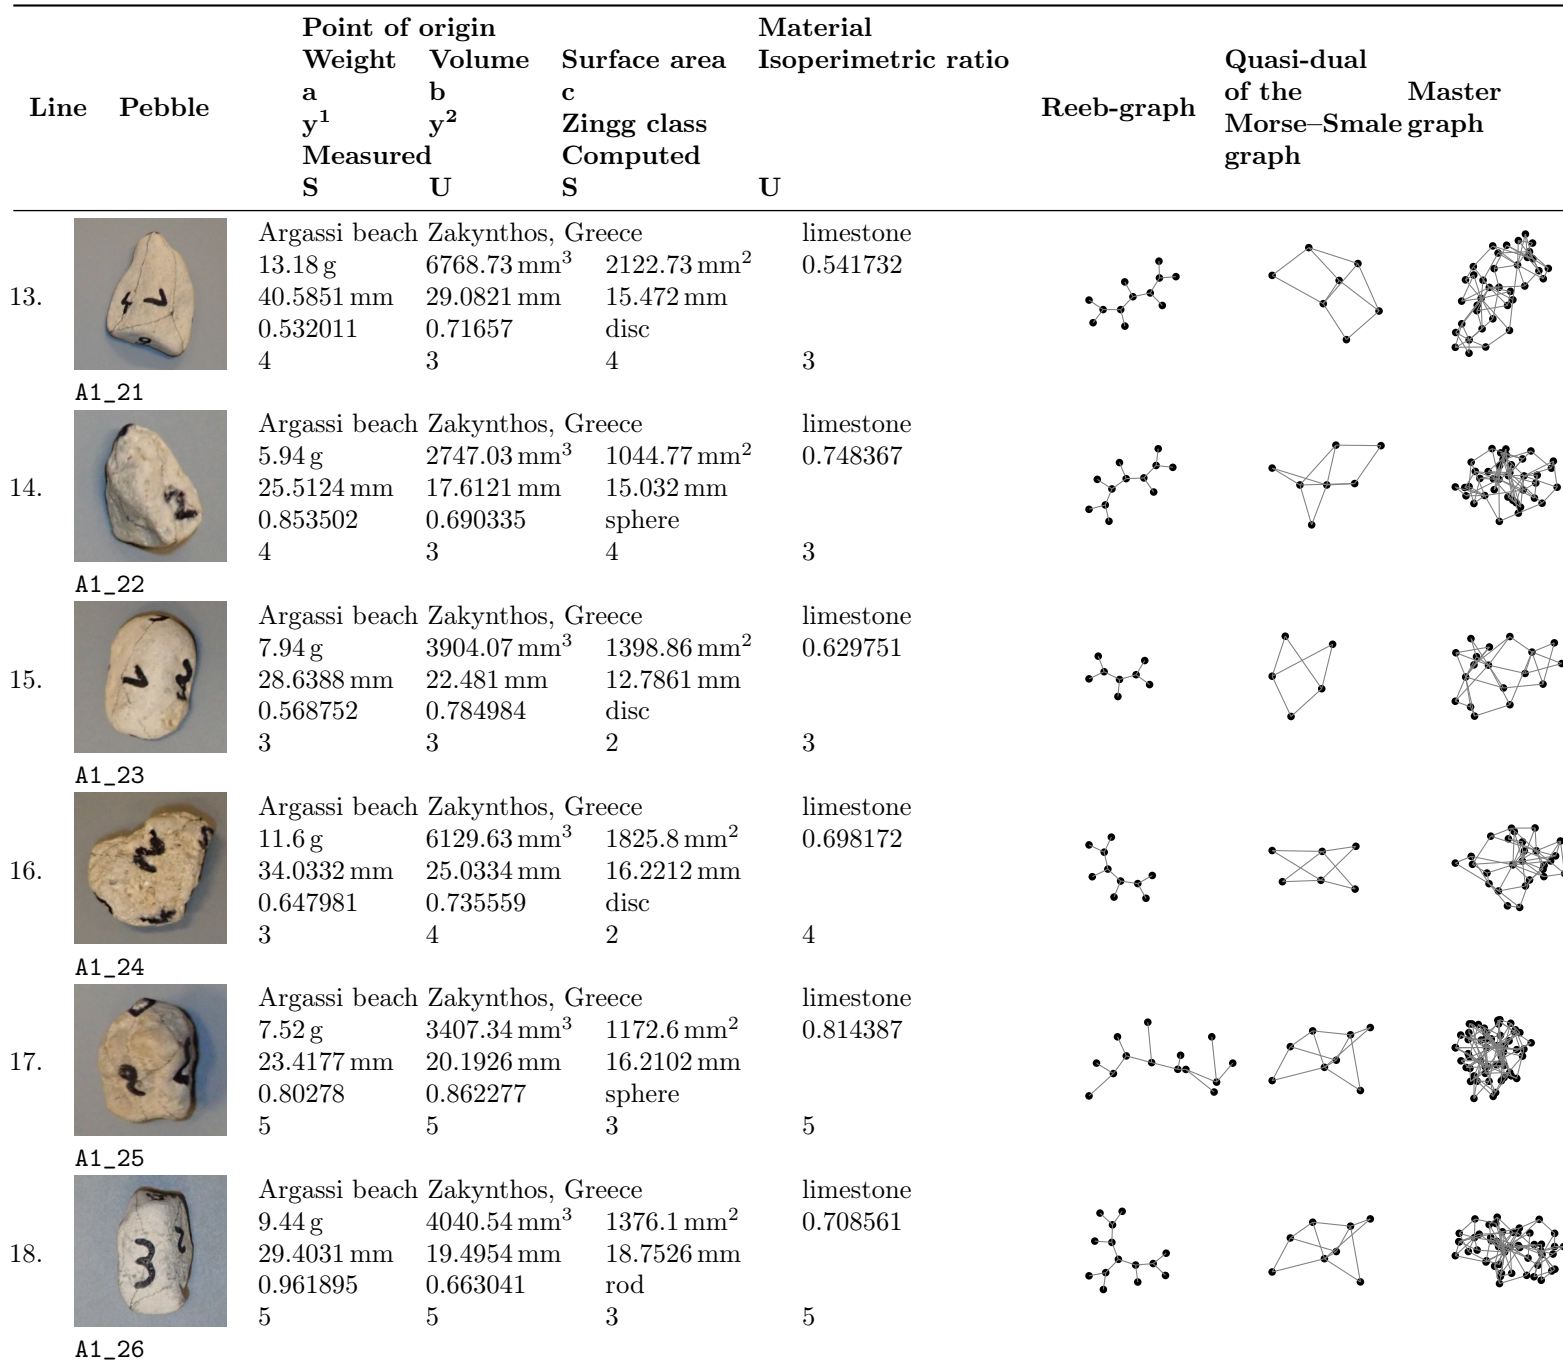 |
| A1_26 |                                                                                     |                                                         |                                                                             |                                                     |                                |                                                                                       |                                                                                       |                                                                                       |

| Line | Pebble                                                                              | Point of origin                                        |                                                                             |                                                                  | Material | Reeb-graph                                                                            | Quasi-dual<br>of the<br>Morse–Smale<br>graph                                          | Master<br>graph                                                                       |
|------|-------------------------------------------------------------------------------------|--------------------------------------------------------|-----------------------------------------------------------------------------|------------------------------------------------------------------|----------|---------------------------------------------------------------------------------------|---------------------------------------------------------------------------------------|---------------------------------------------------------------------------------------|
|      |                                                                                     | Weight                                                 | Volume                                                                      | Surface area                                                     |          |                                                                                       |                                                                                       |                                                                                       |
|      |                                                                                     | a                                                      | b                                                                           | c                                                                |          |                                                                                       |                                                                                       |                                                                                       |
|      |                                                                                     | y <sup>1</sup><br>Measured<br>S                        | y <sup>2</sup><br>U                                                         | Zingg class<br>Computed<br>S                                     |          |                                                                                       |                                                                                       |                                                                                       |
| 19.  | 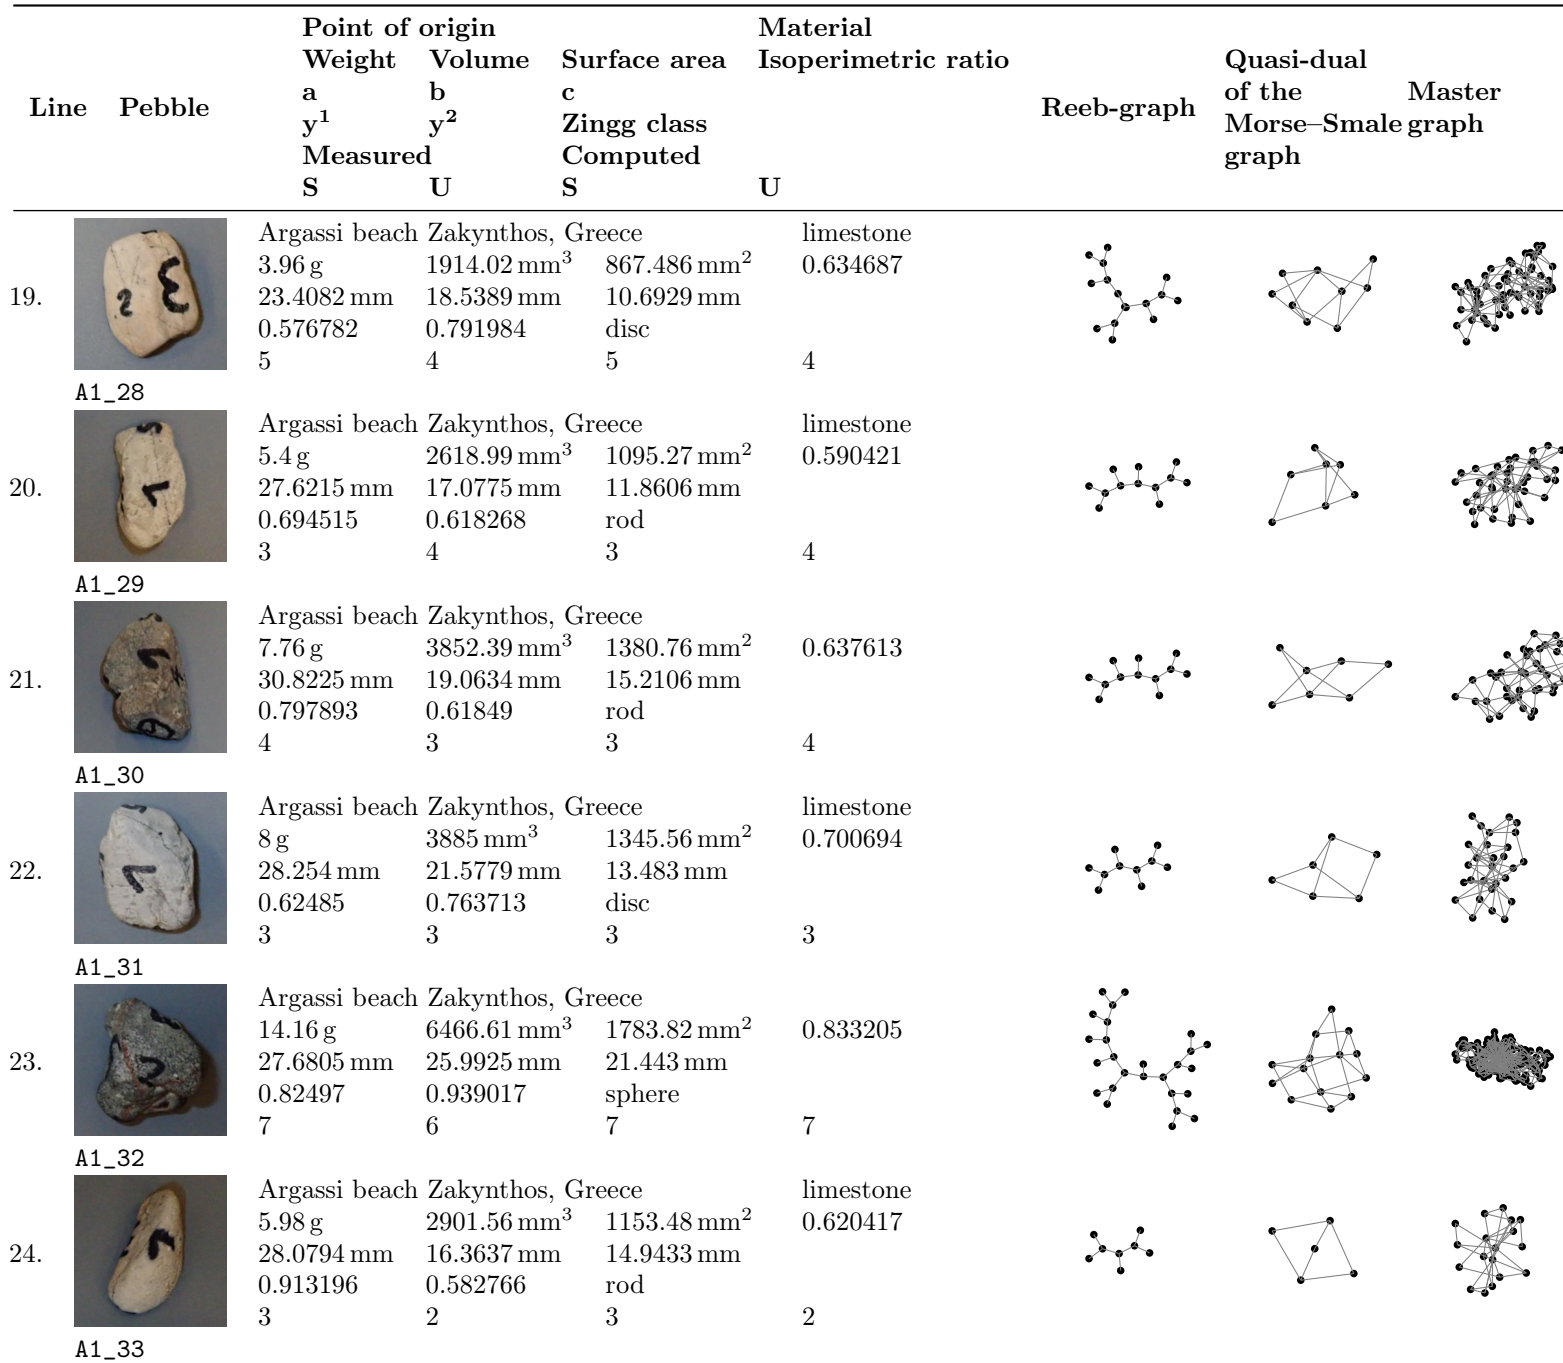   | Argassi beach<br>3.96 g<br>23.4082 mm<br>0.576782<br>5 | Zakynthos, Greece<br>1914.02 mm <sup>3</sup><br>18.5389 mm<br>0.791984<br>4 | limestone<br>867.486 mm <sup>2</sup><br>10.6929 mm<br>disc<br>5  | 0.634687 | 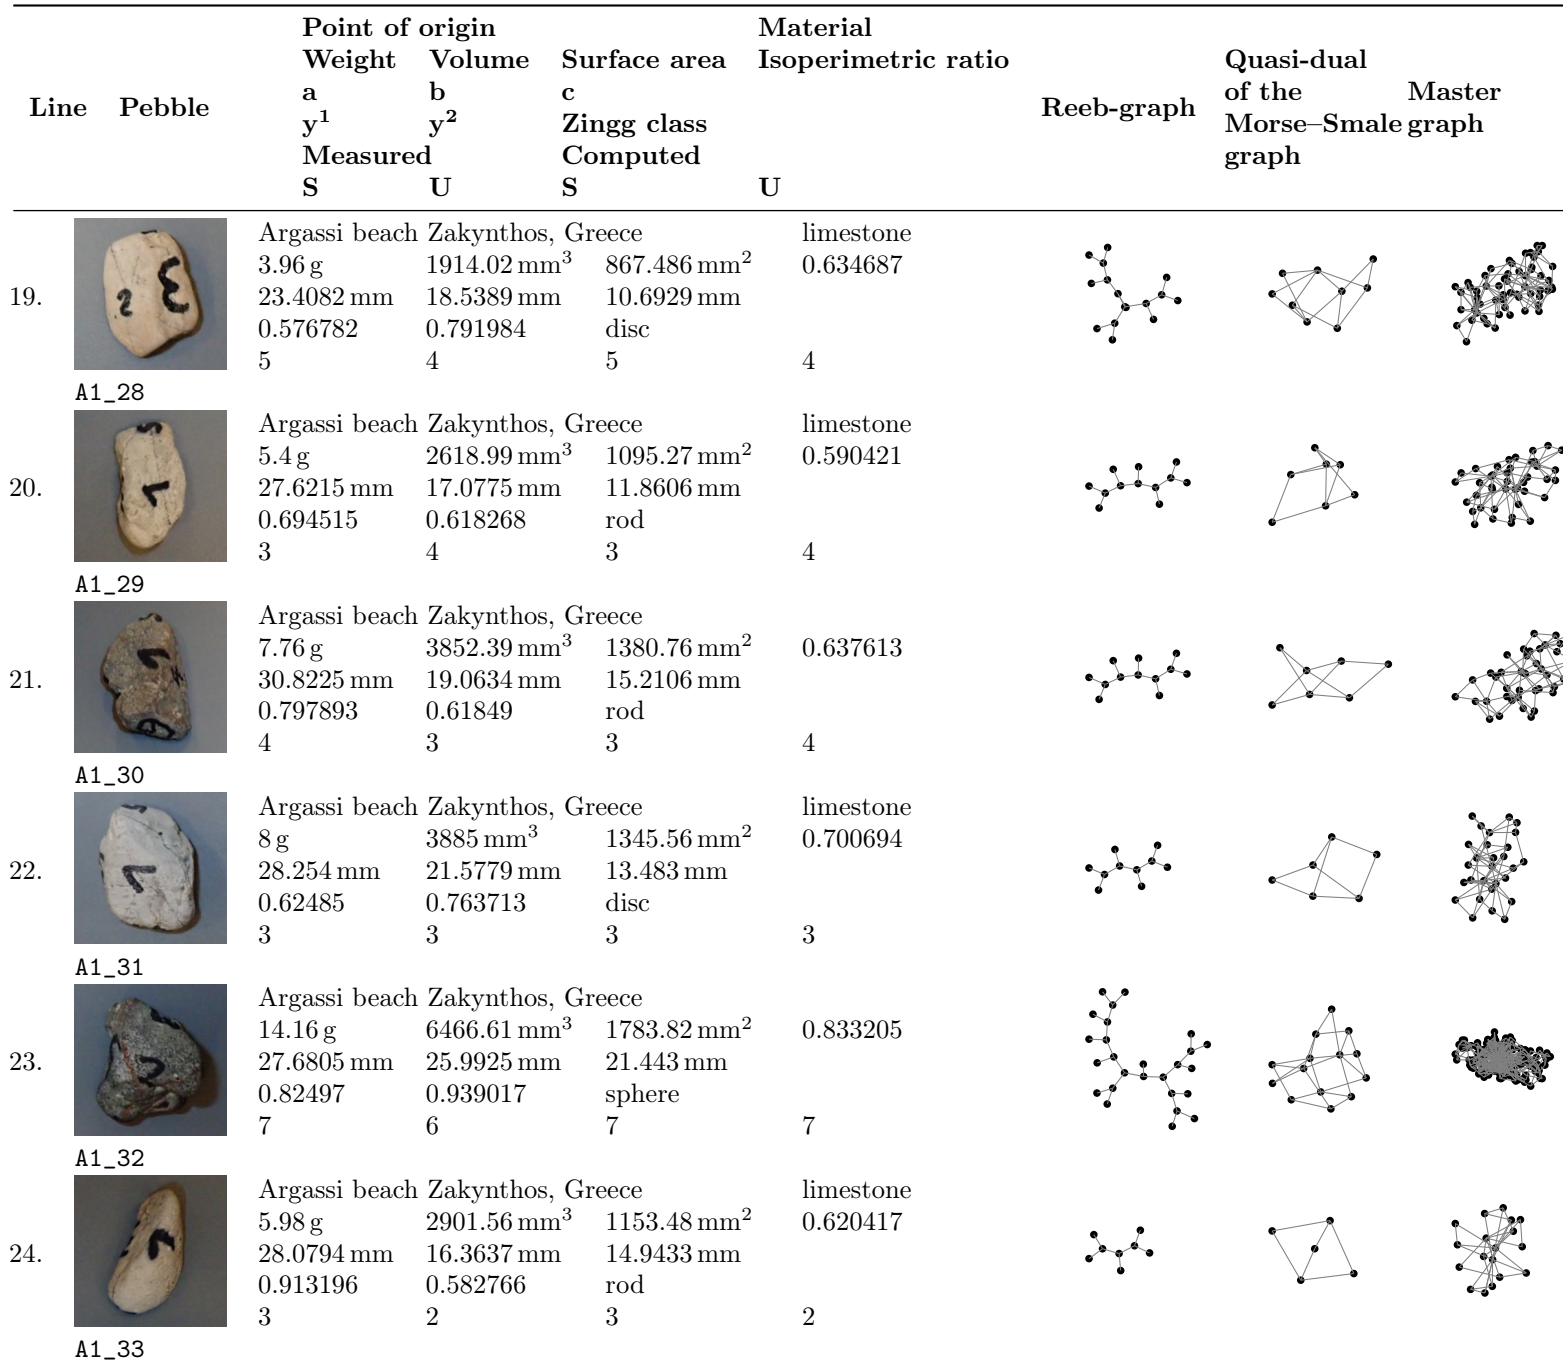   | 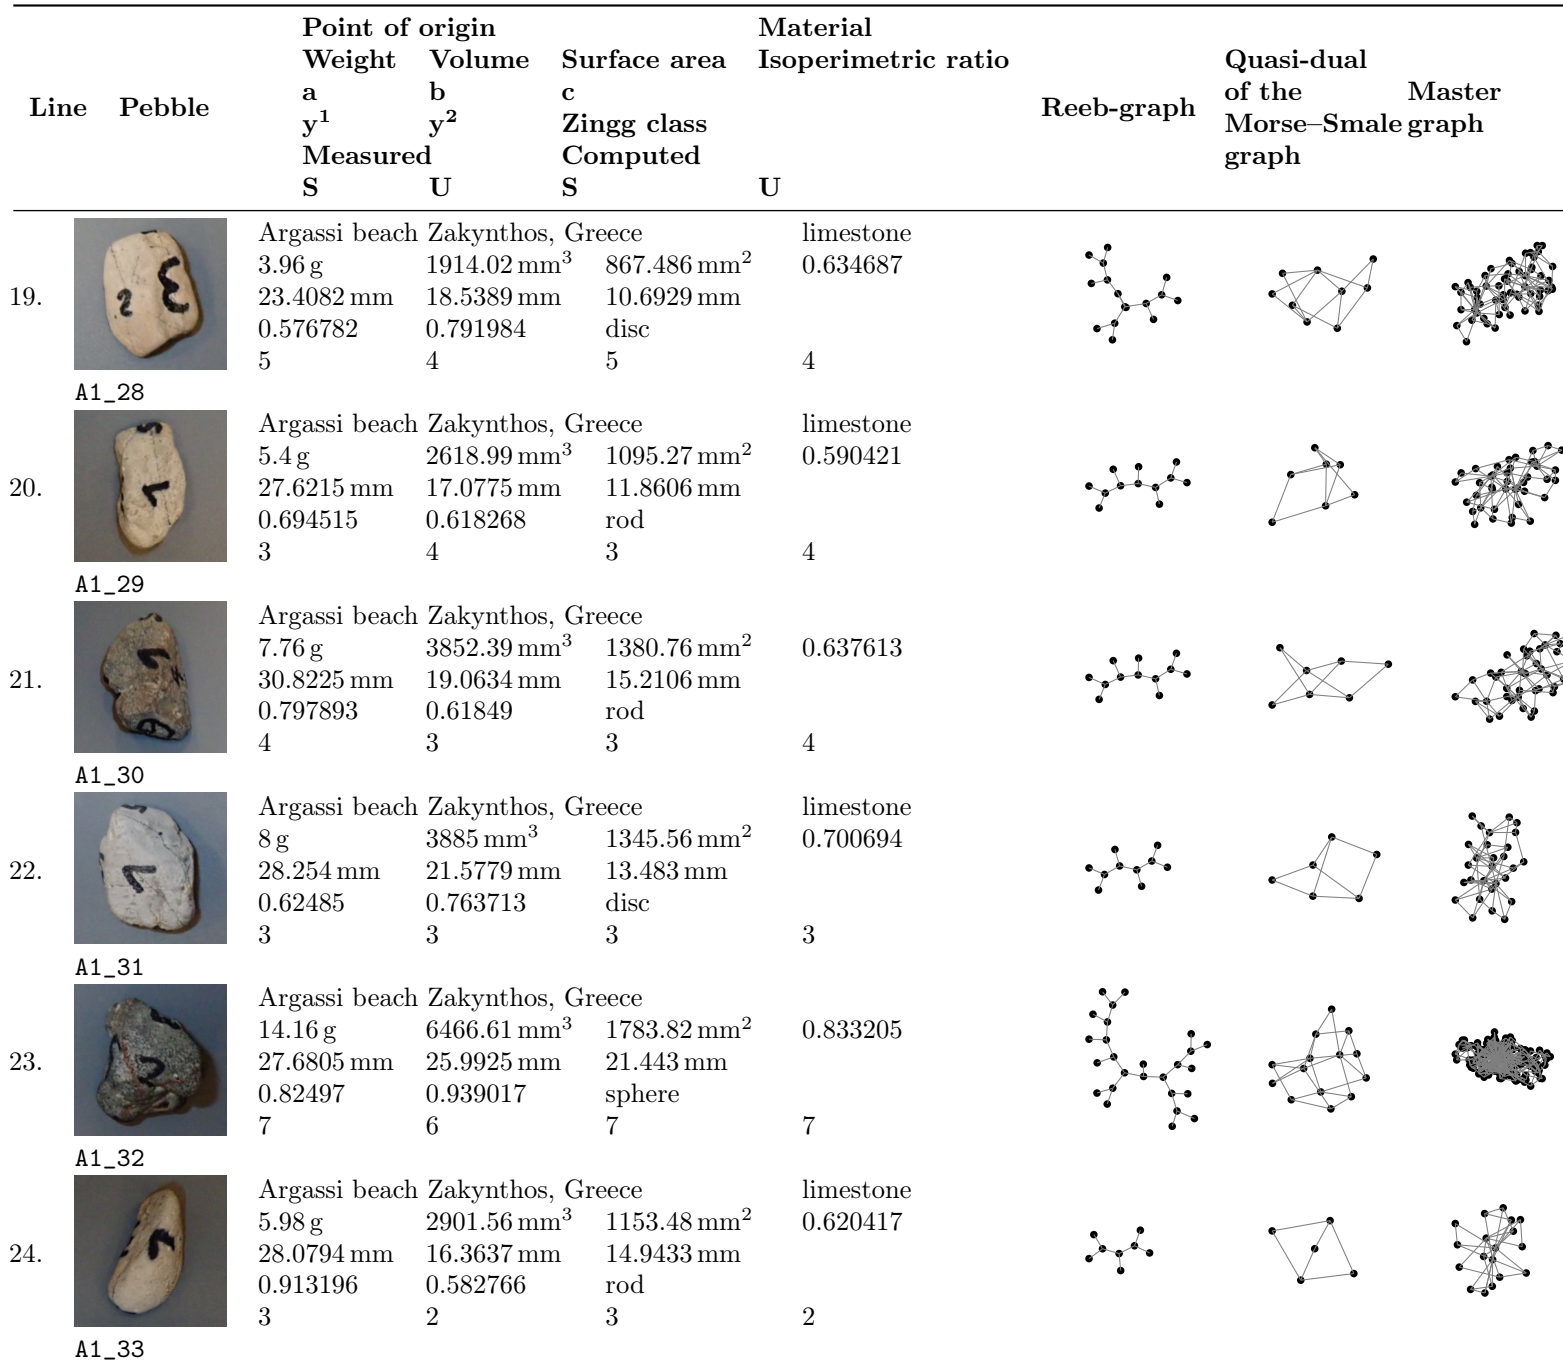   | 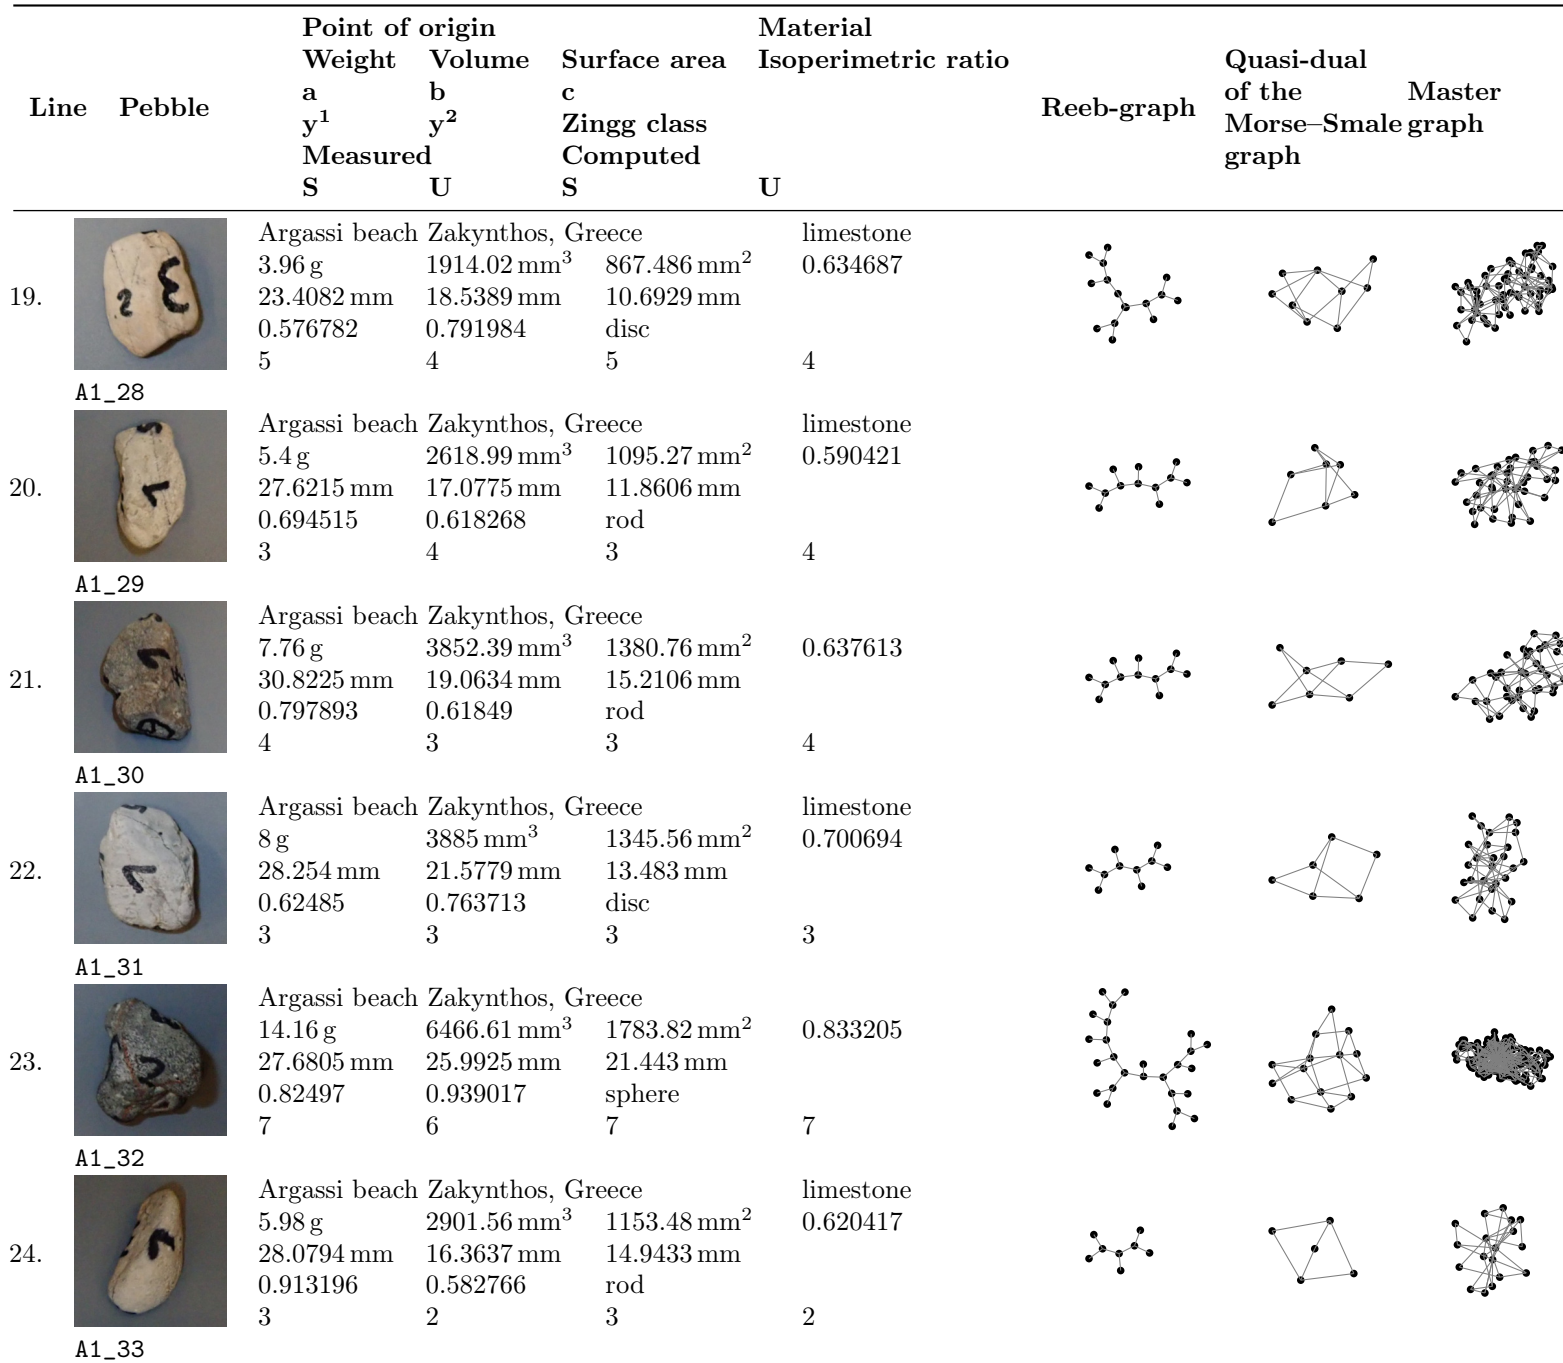   |
|      | A1_28                                                                               |                                                        |                                                                             |                                                                  |          |                                                                                       |                                                                                       |                                                                                       |
| 20.  | 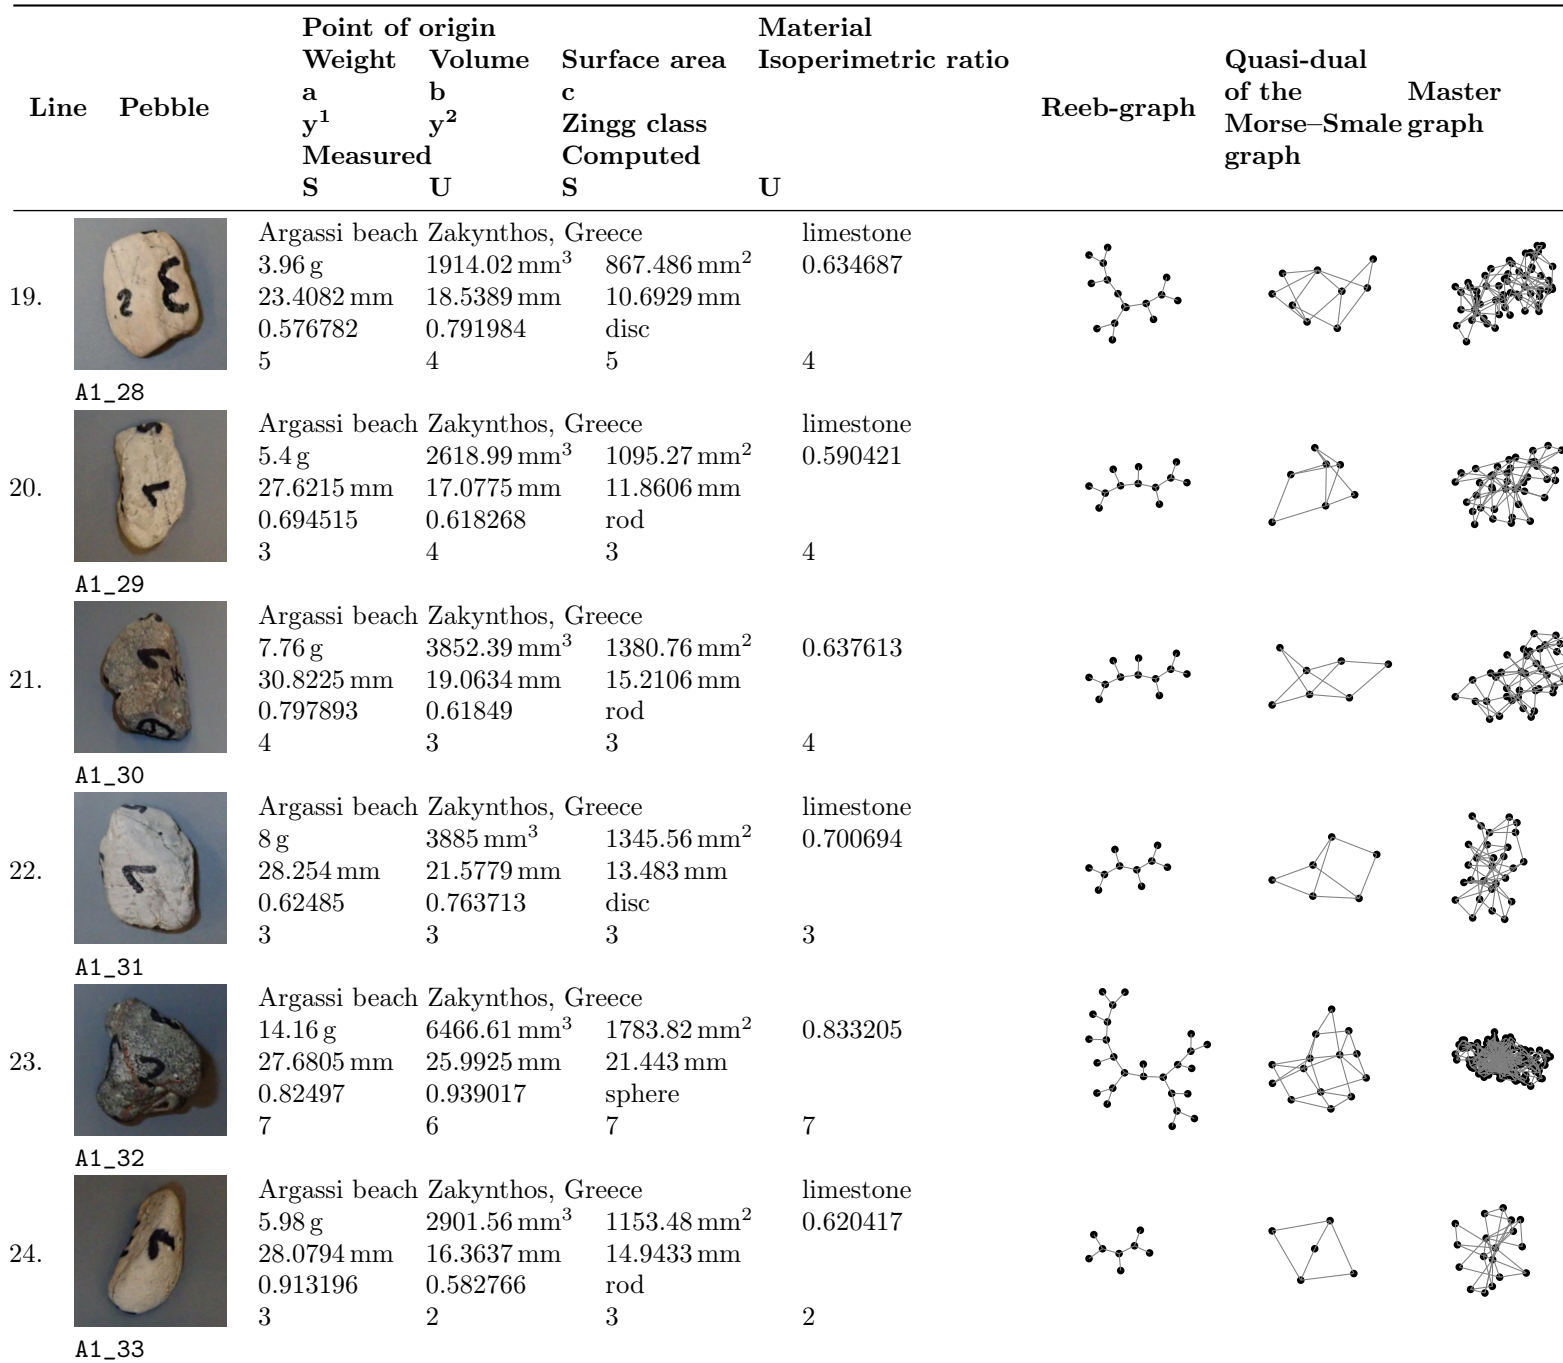   | Argassi beach<br>5.4 g<br>27.6215 mm<br>0.694515<br>3  | Zakynthos, Greece<br>2618.99 mm <sup>3</sup><br>17.0775 mm<br>0.618268<br>4 | limestone<br>1095.27 mm <sup>2</sup><br>11.8606 mm<br>rod<br>3   | 0.590421 | 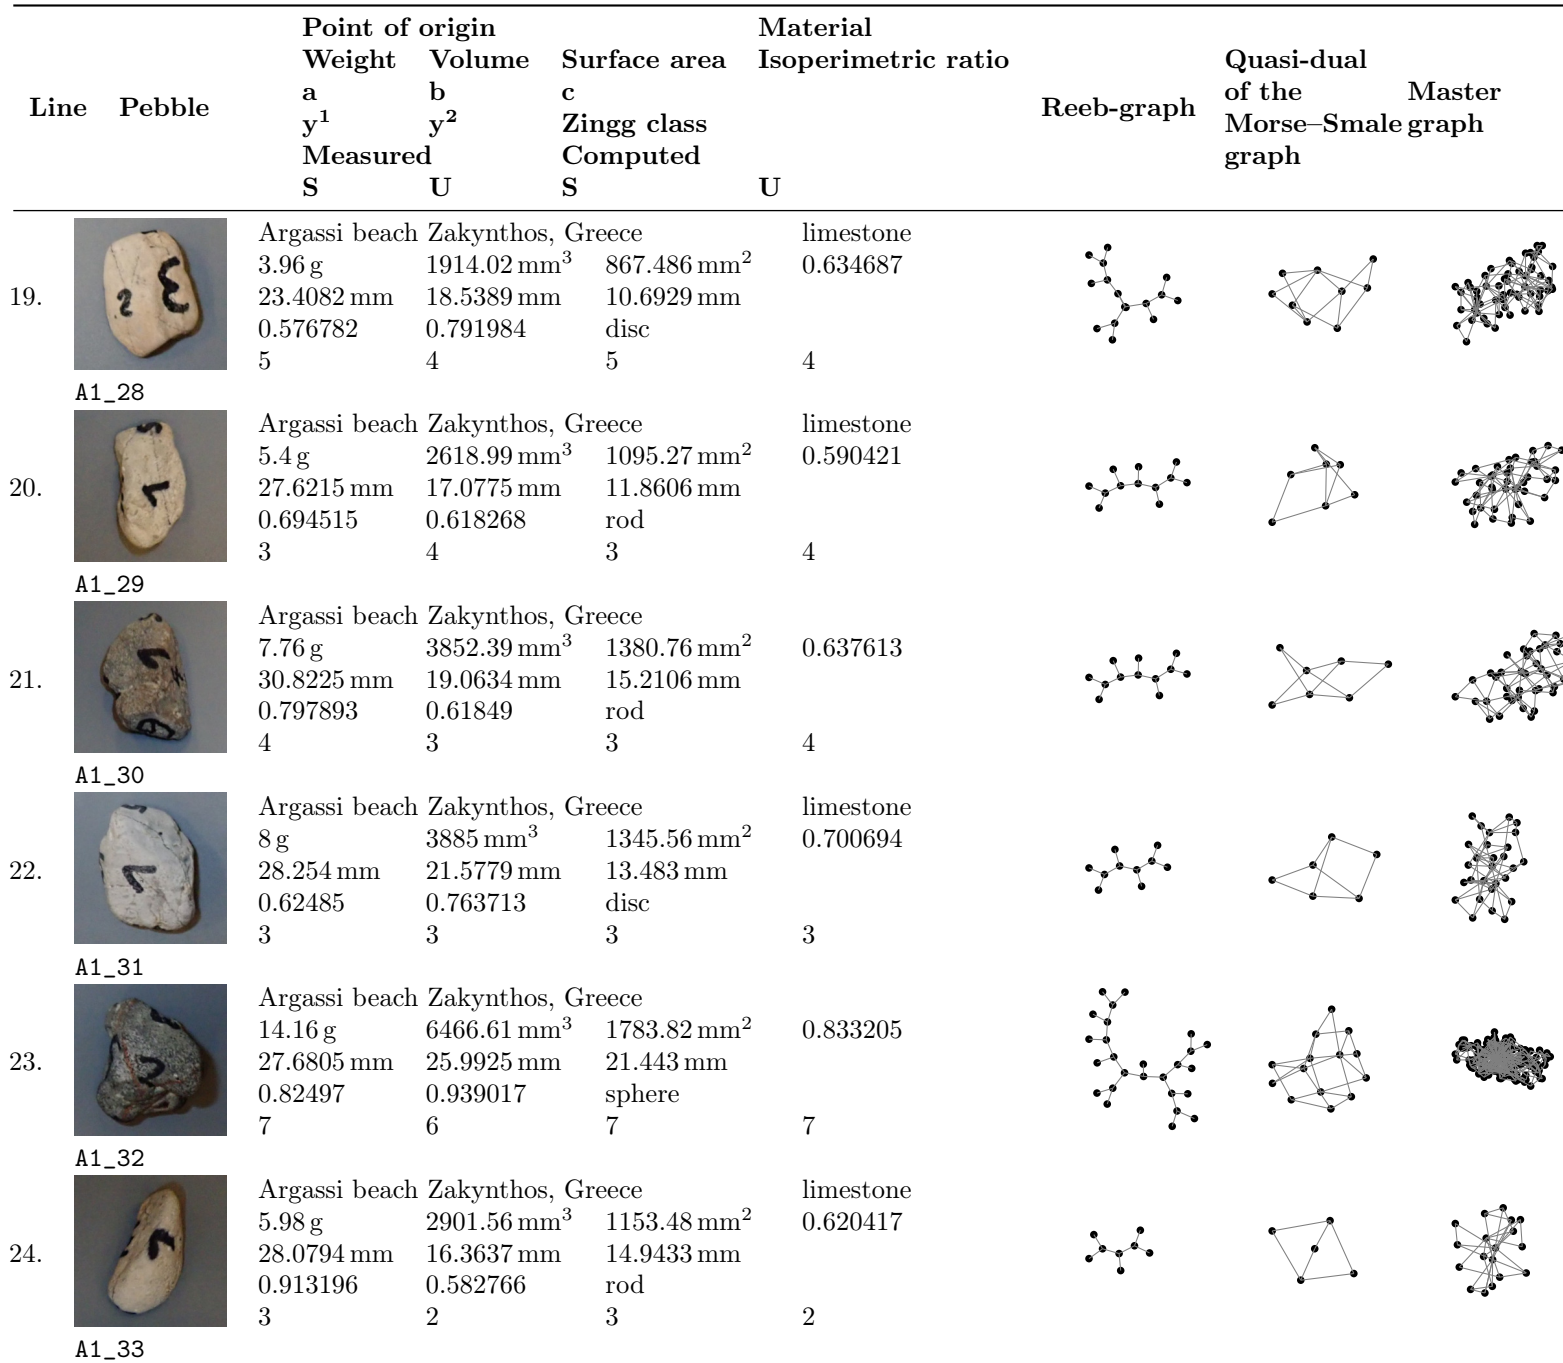   | 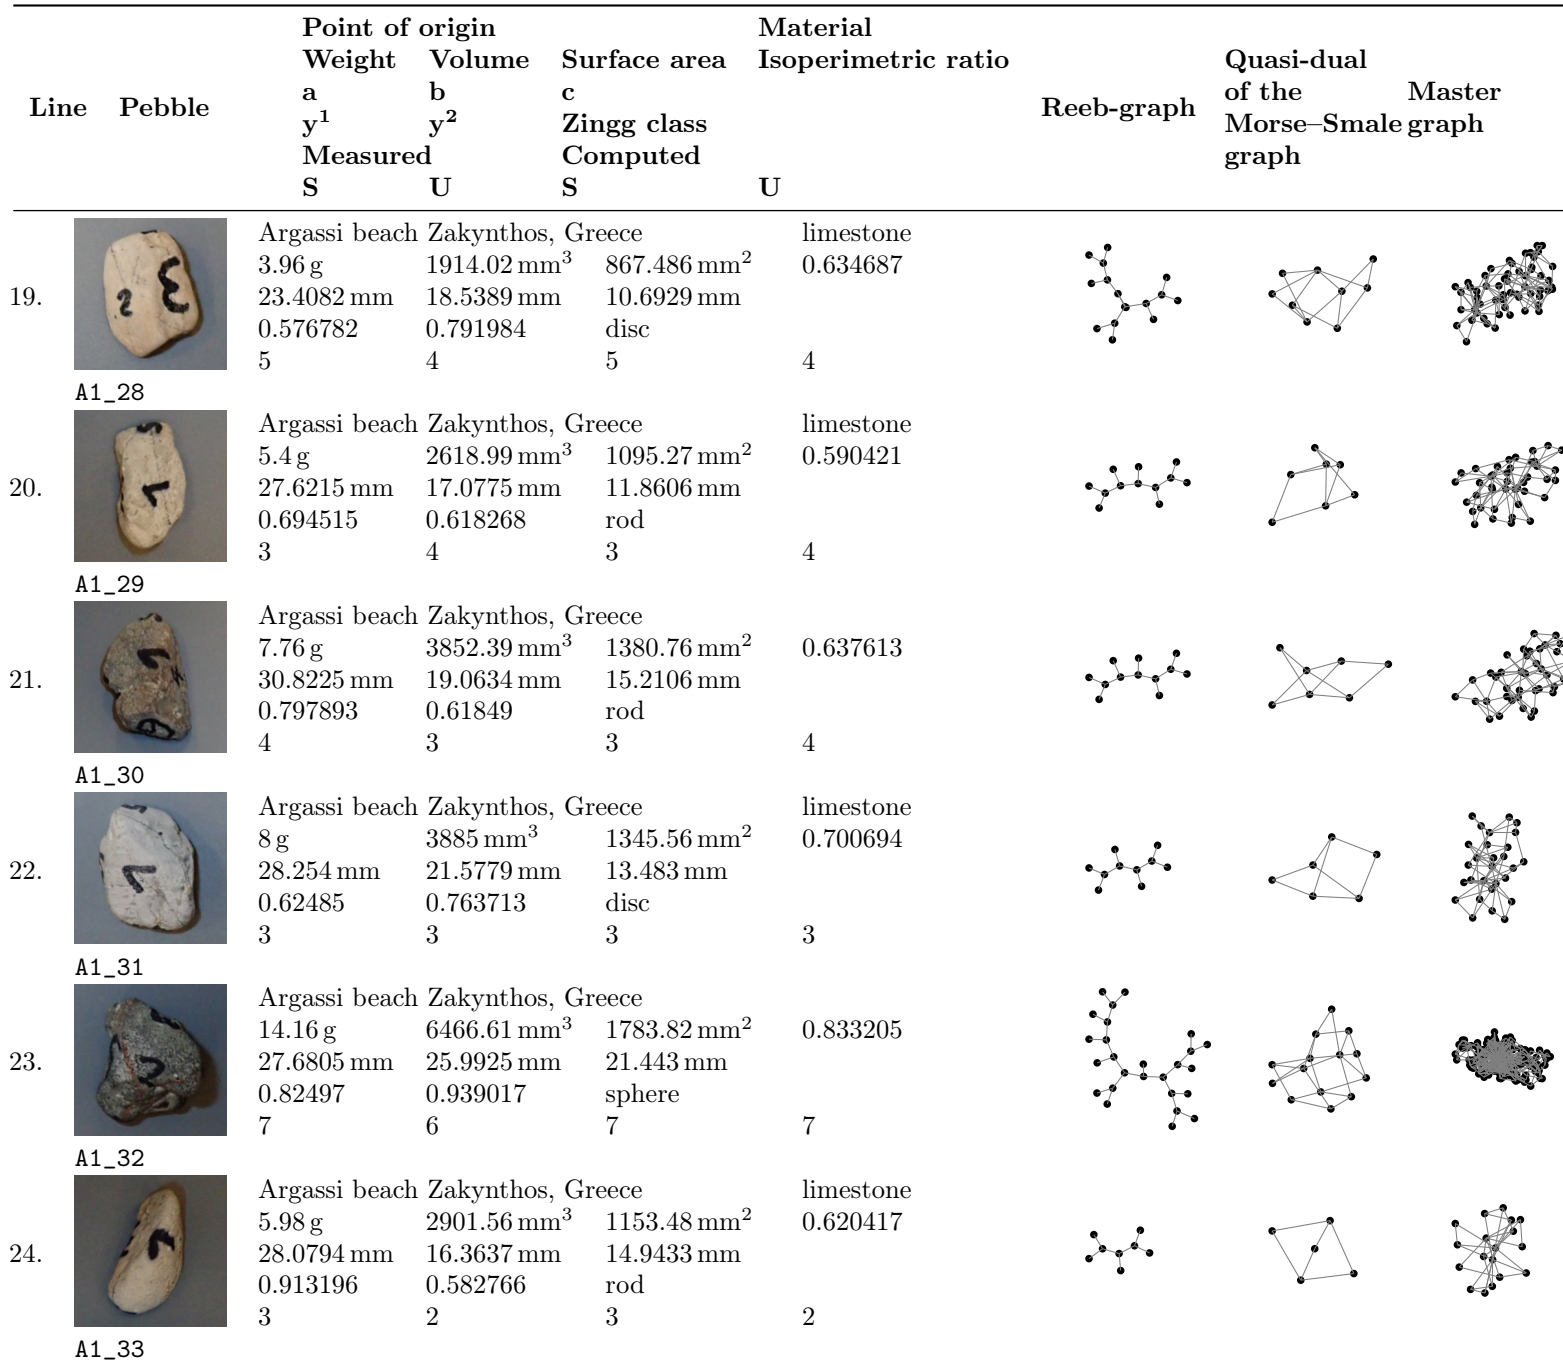   | 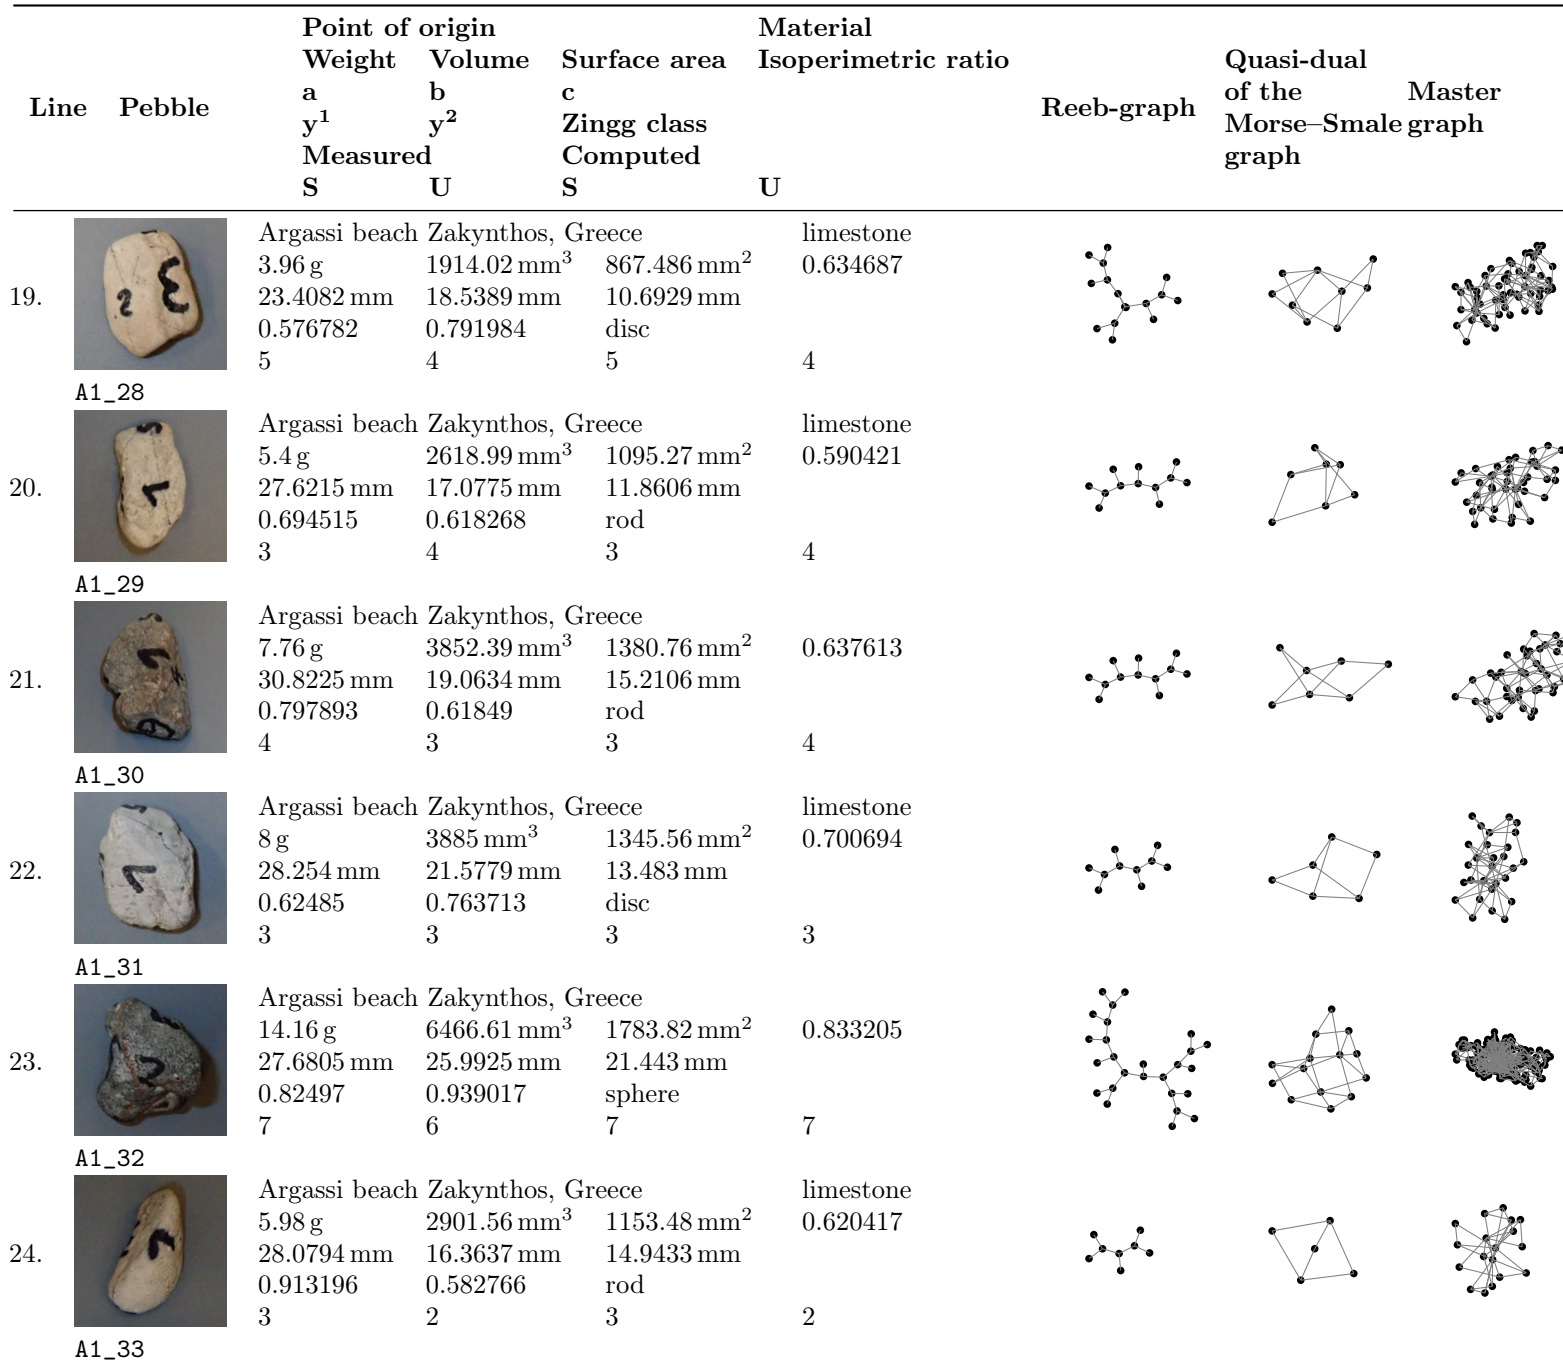   |
|      | A1_29                                                                               |                                                        |                                                                             |                                                                  |          |                                                                                       |                                                                                       |                                                                                       |
| 21.  | 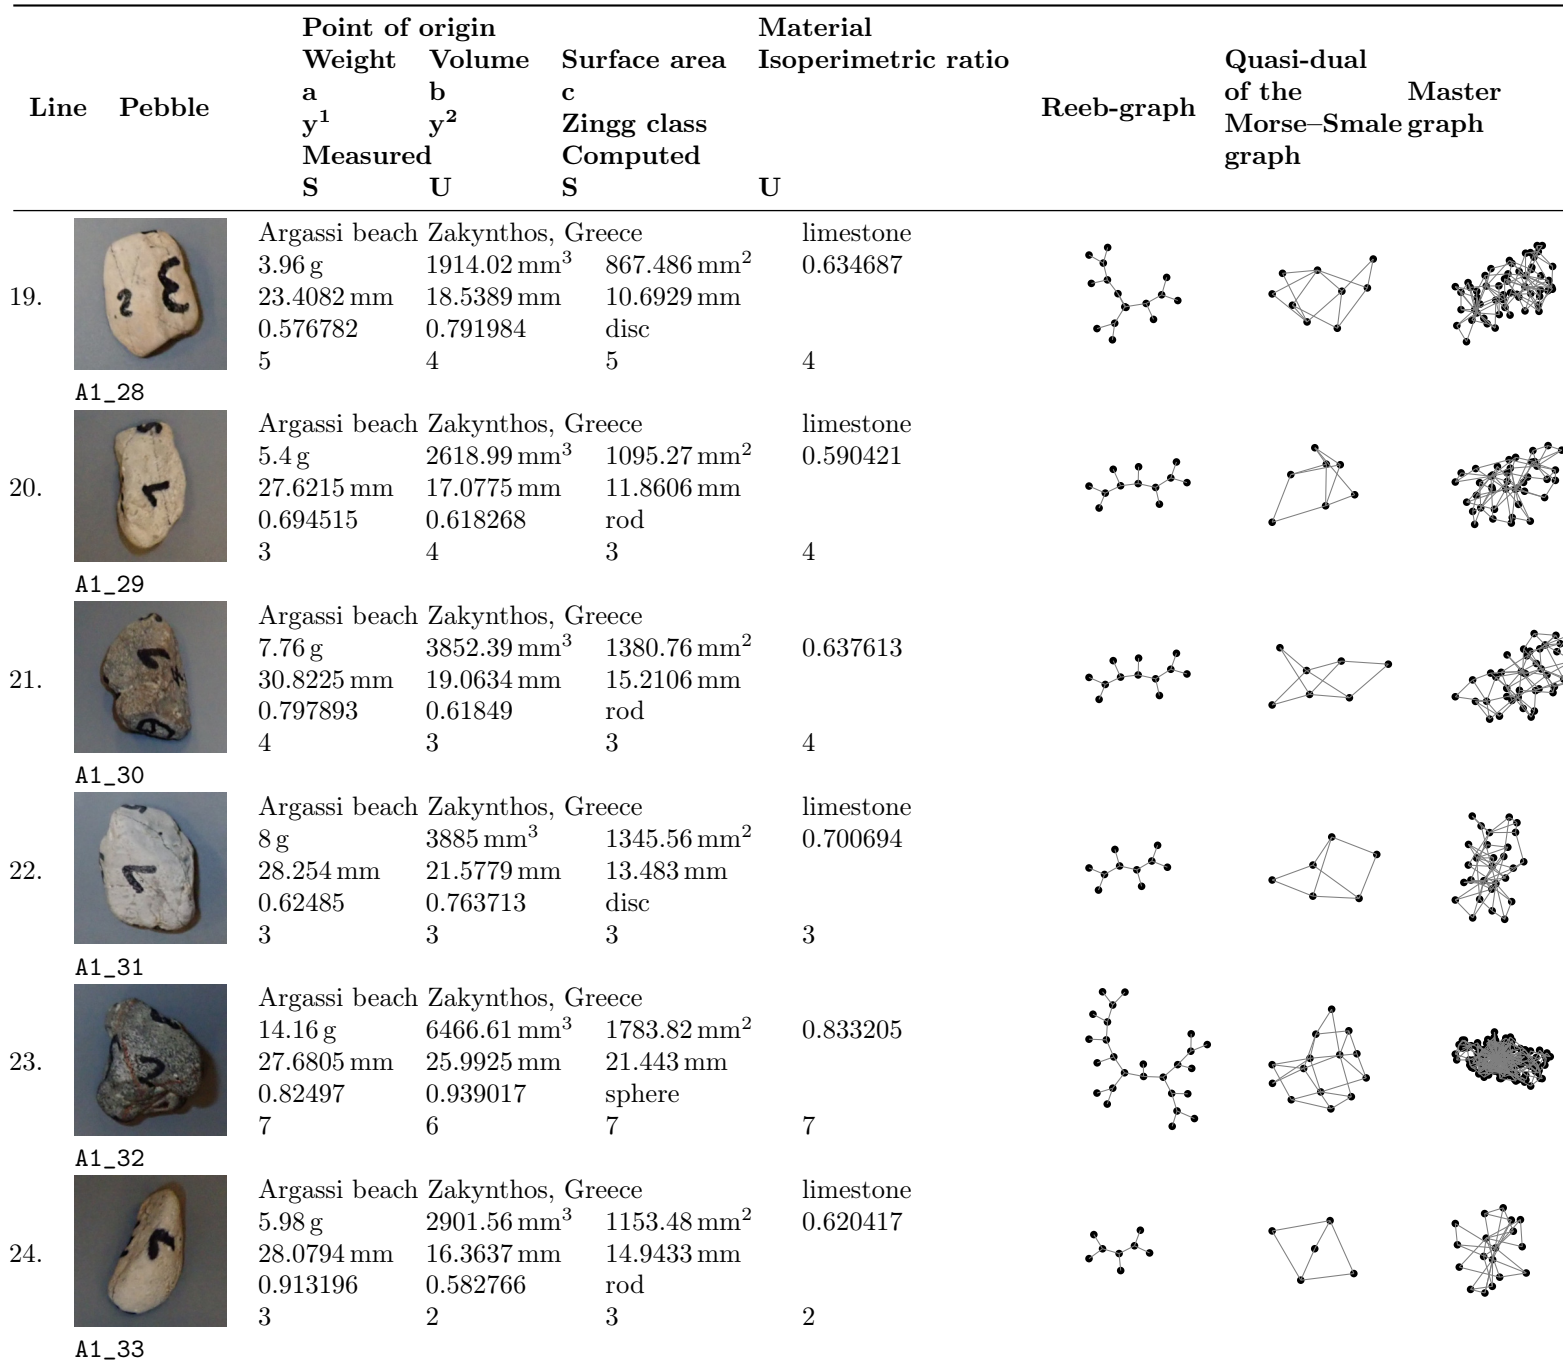   | Argassi beach<br>7.76 g<br>30.8225 mm<br>0.797893<br>4 | Zakynthos, Greece<br>3852.39 mm <sup>3</sup><br>19.0634 mm<br>0.61849<br>3  | limestone<br>1380.76 mm <sup>2</sup><br>15.2106 mm<br>rod<br>3   | 0.637613 | 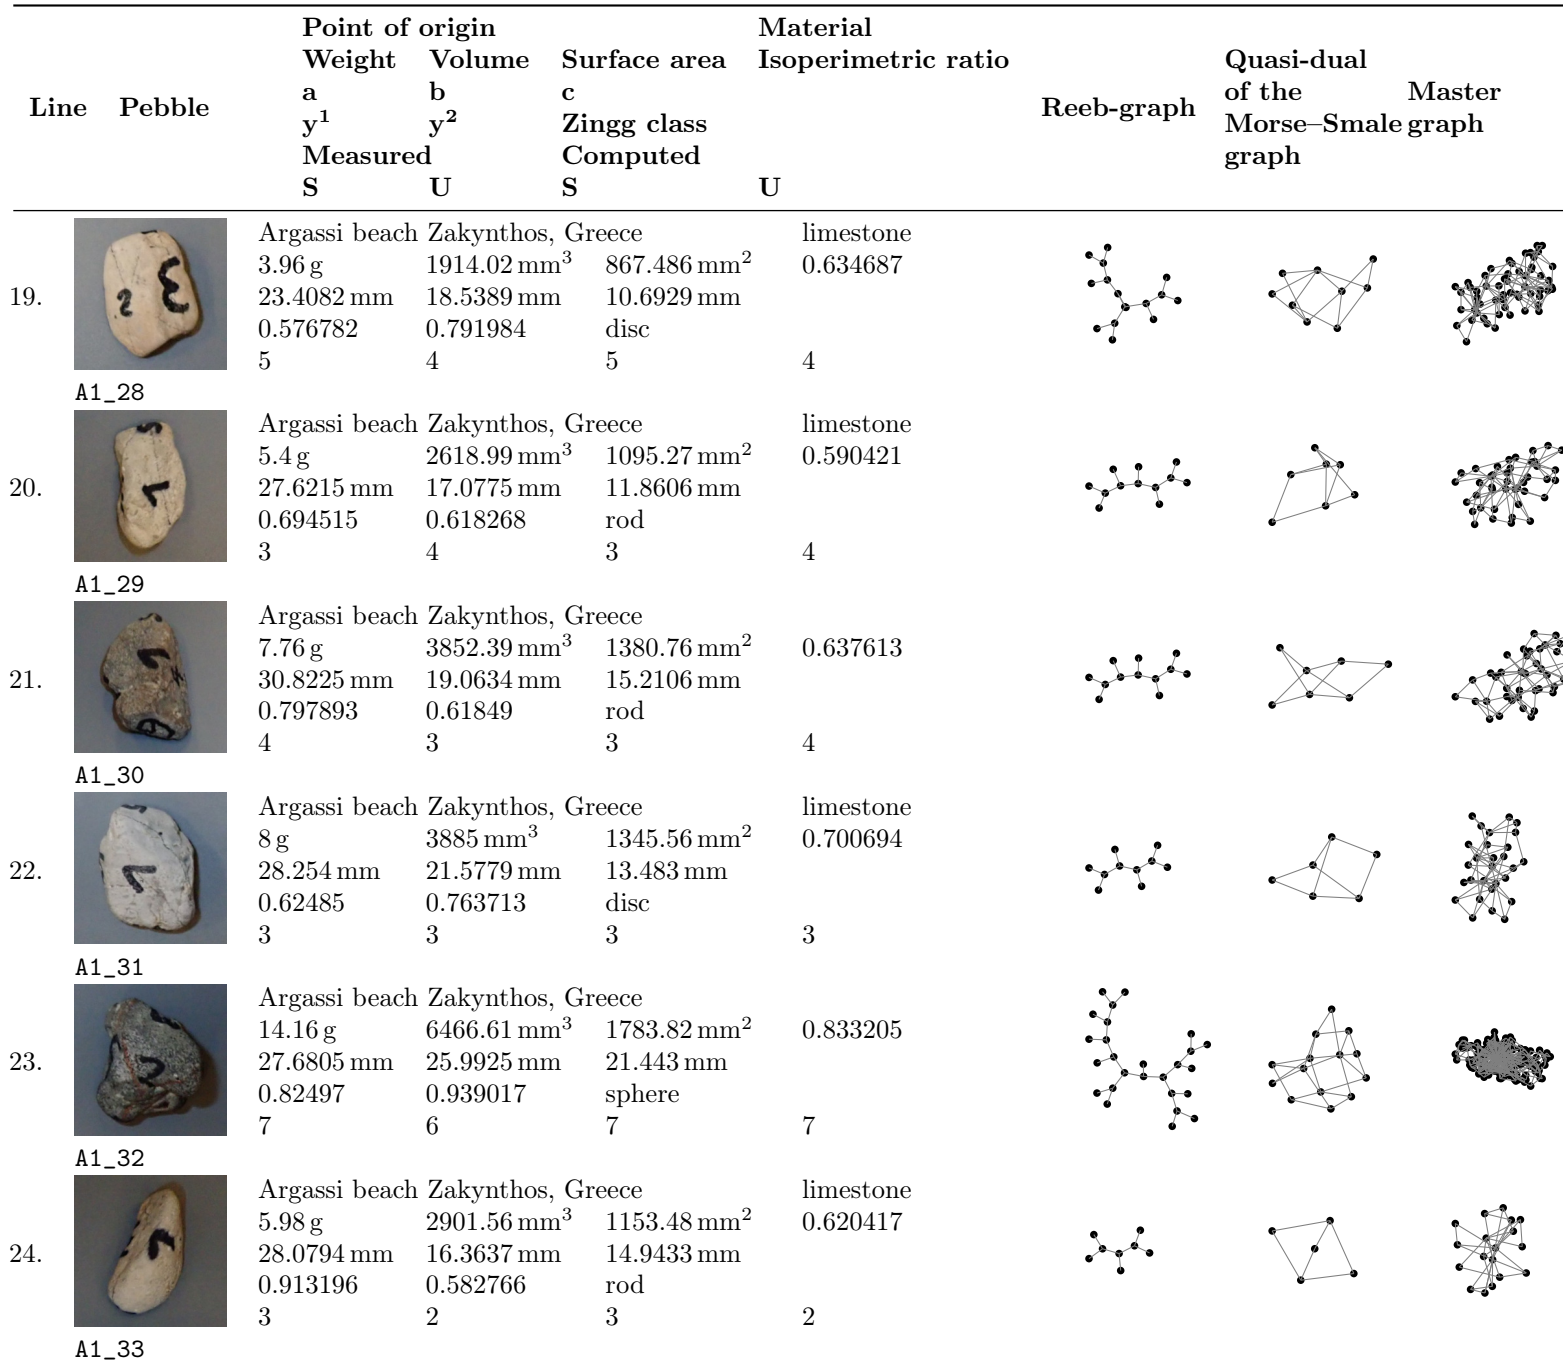   | 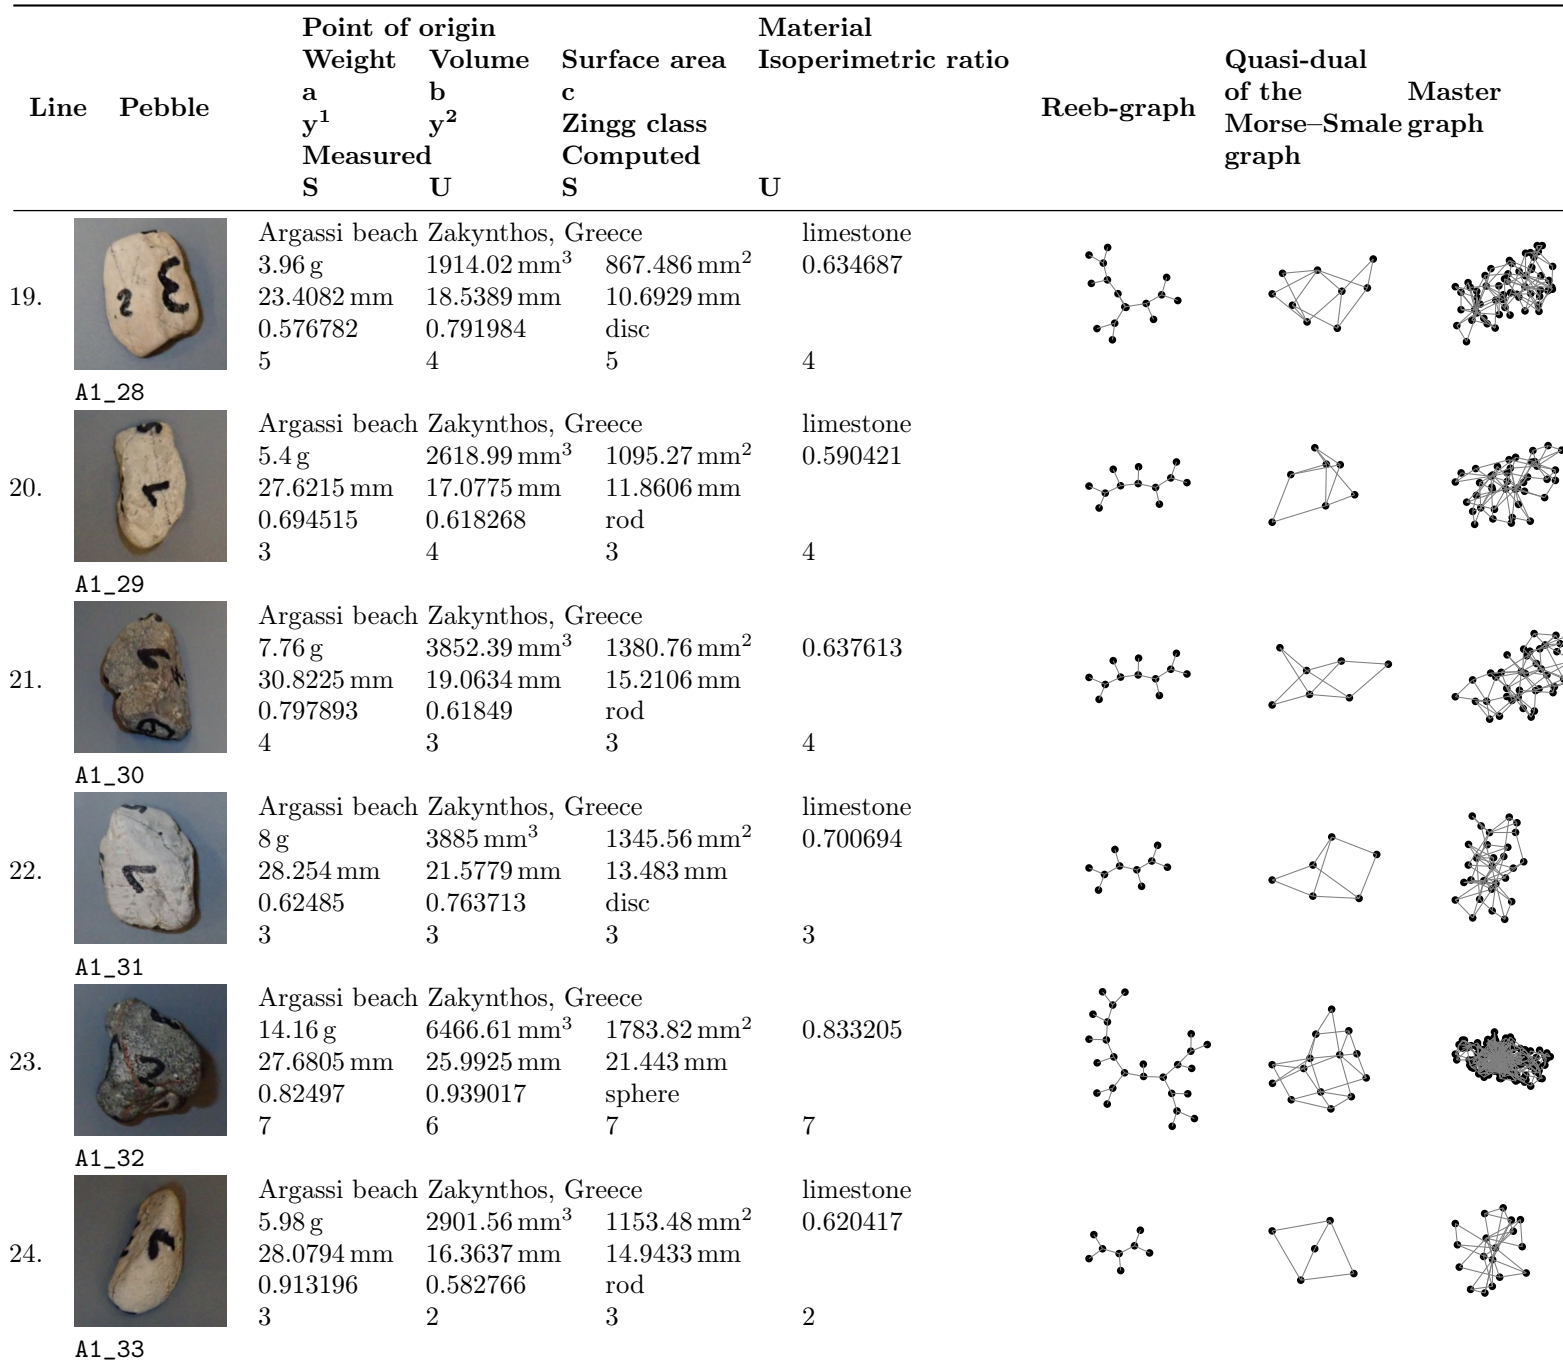   | 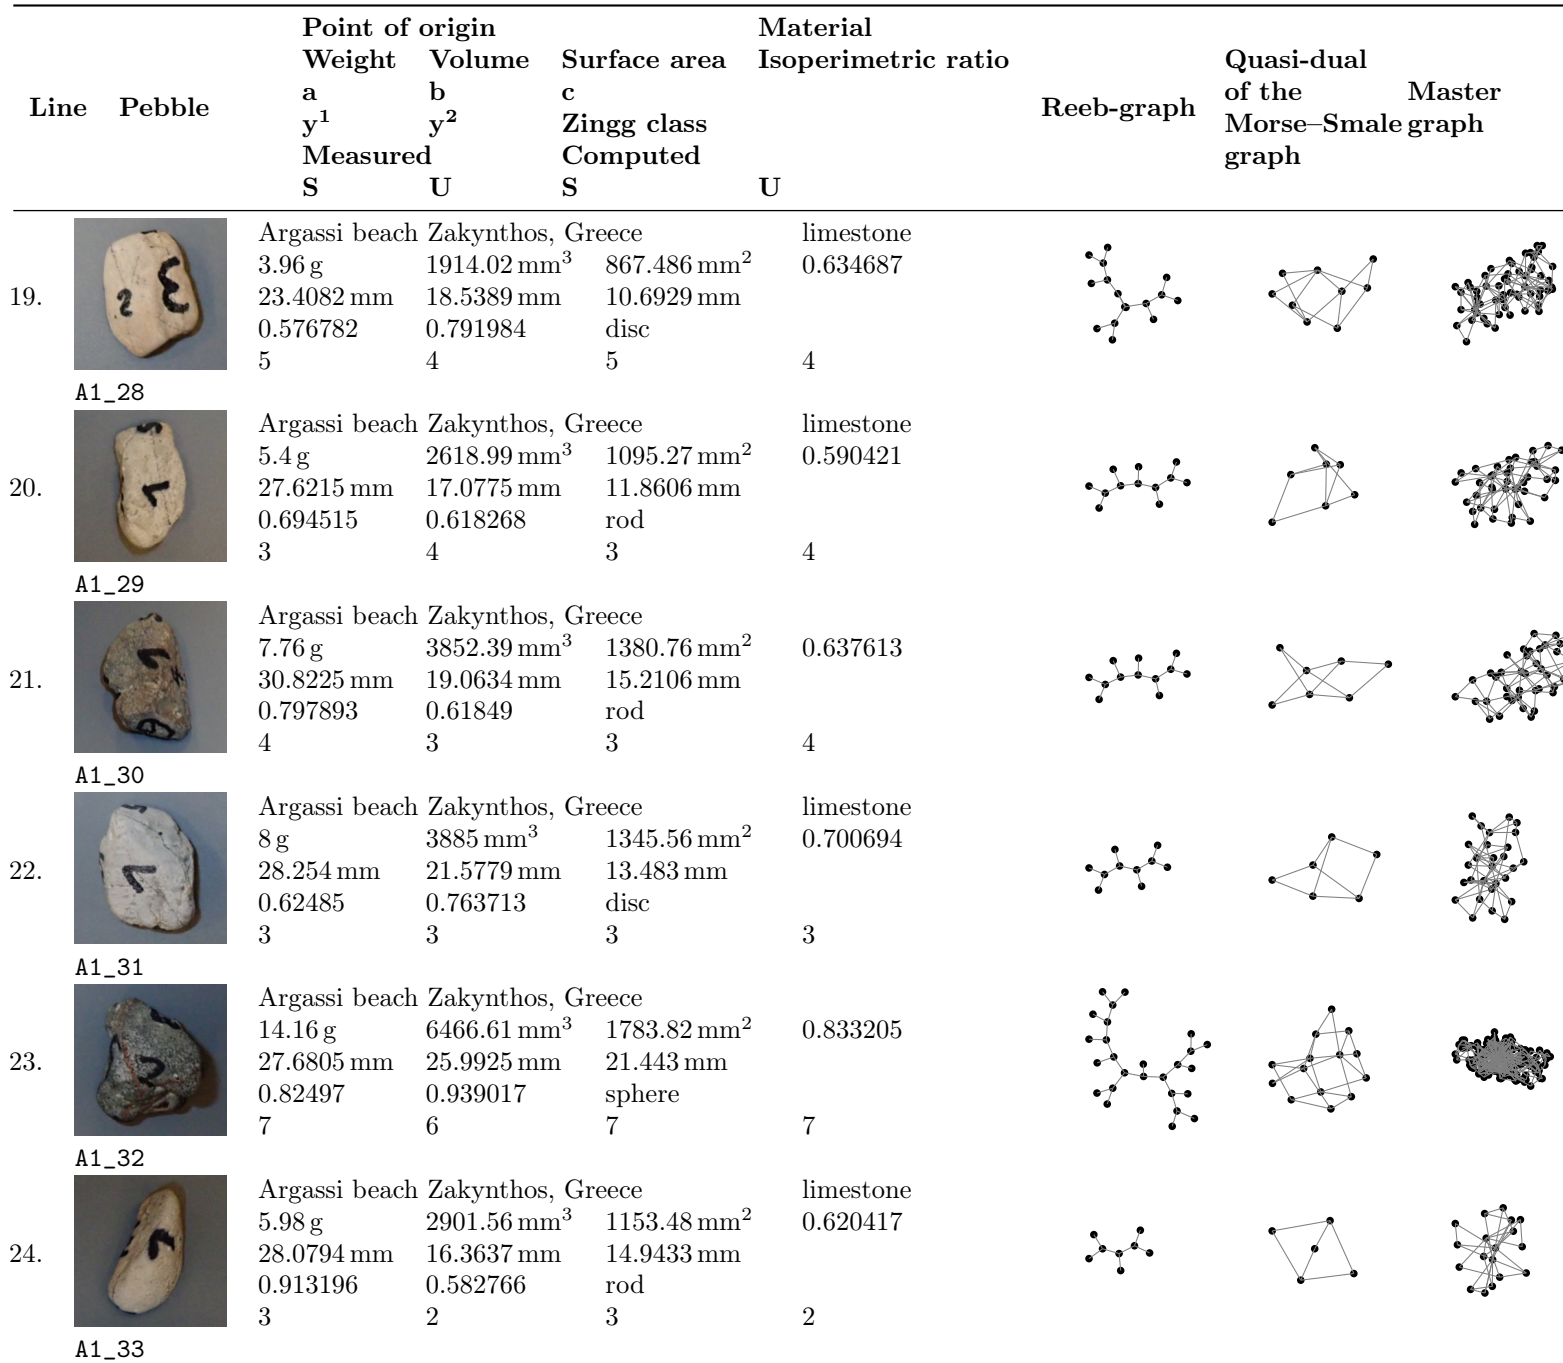   |
|      | A1_30                                                                               |                                                        |                                                                             |                                                                  |          |                                                                                       |                                                                                       |                                                                                       |
| 22.  | 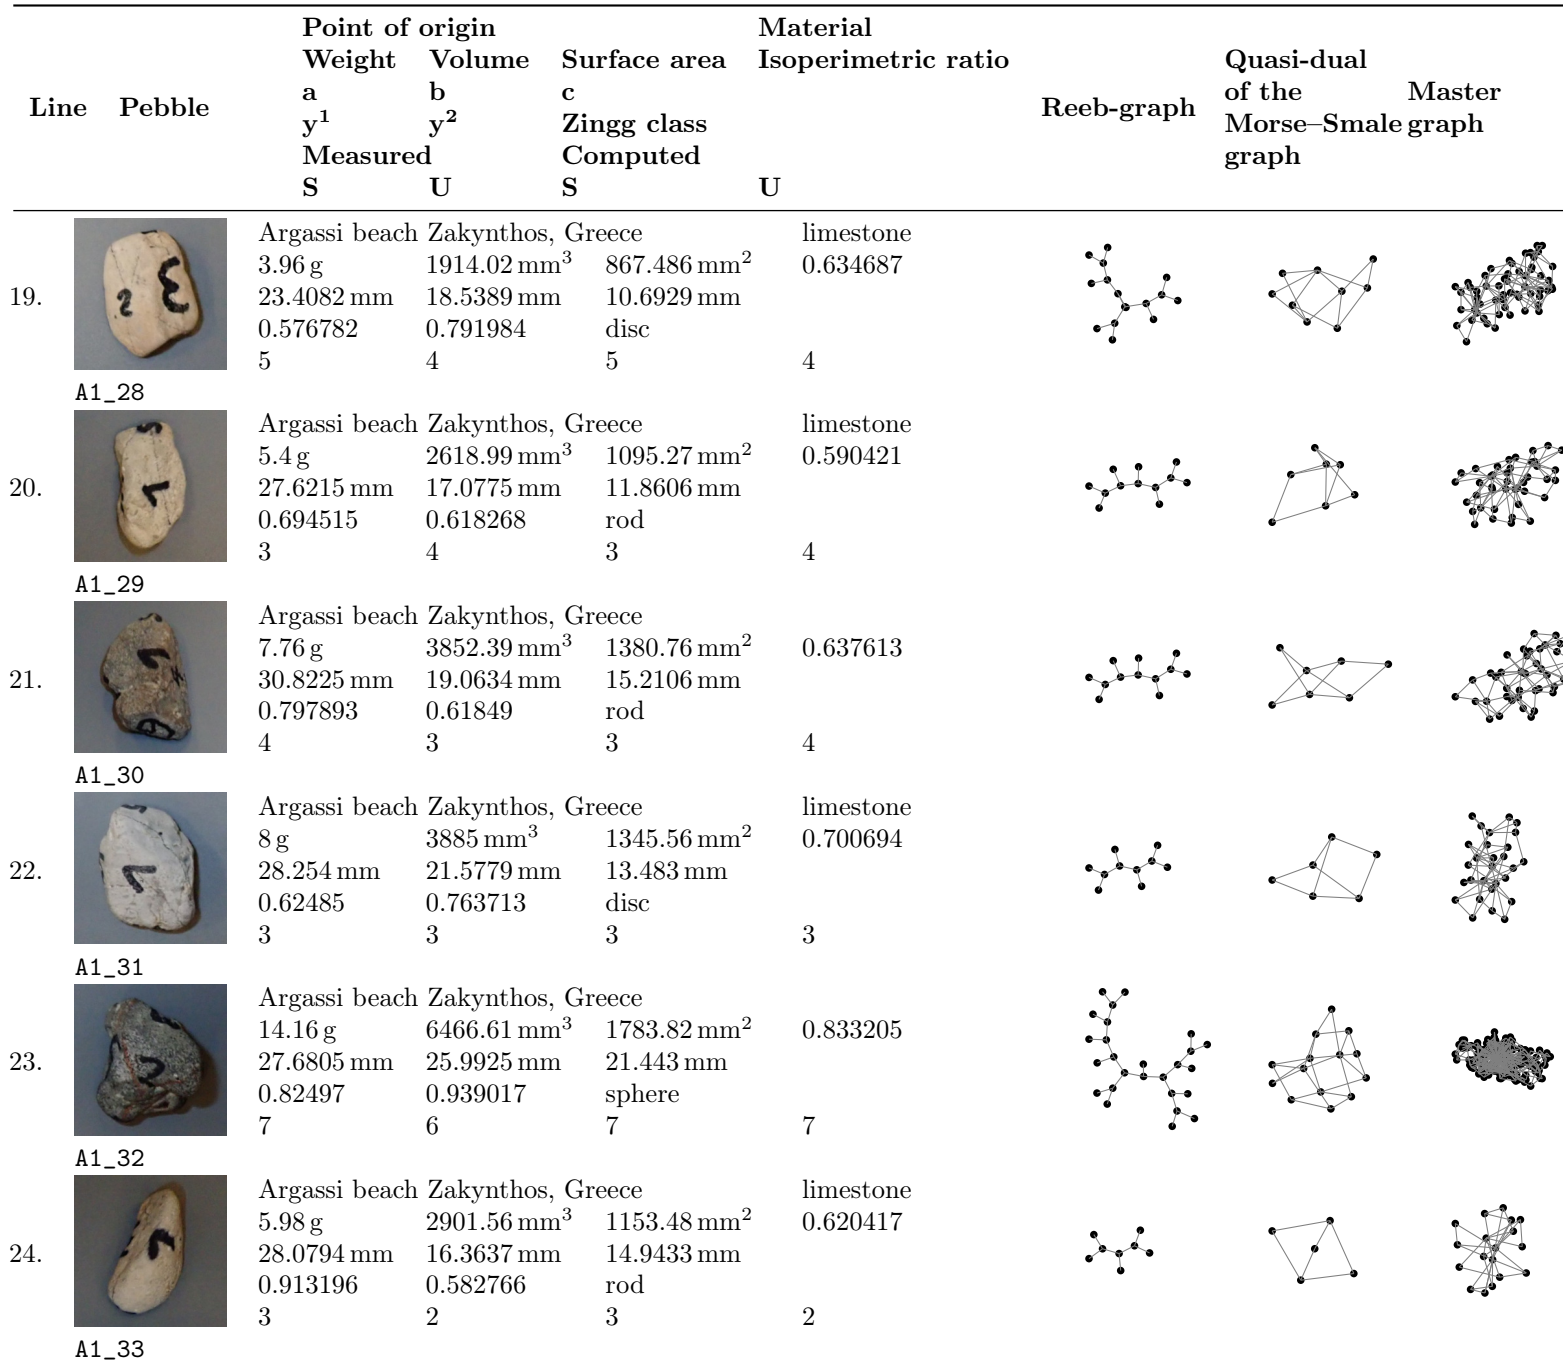  | Argassi beach<br>8 g<br>28.254 mm<br>0.62485<br>3      | Zakynthos, Greece<br>3885 mm <sup>3</sup><br>21.5779 mm<br>0.763713<br>3    | limestone<br>1345.56 mm <sup>2</sup><br>13.483 mm<br>disc<br>3   | 0.700694 | 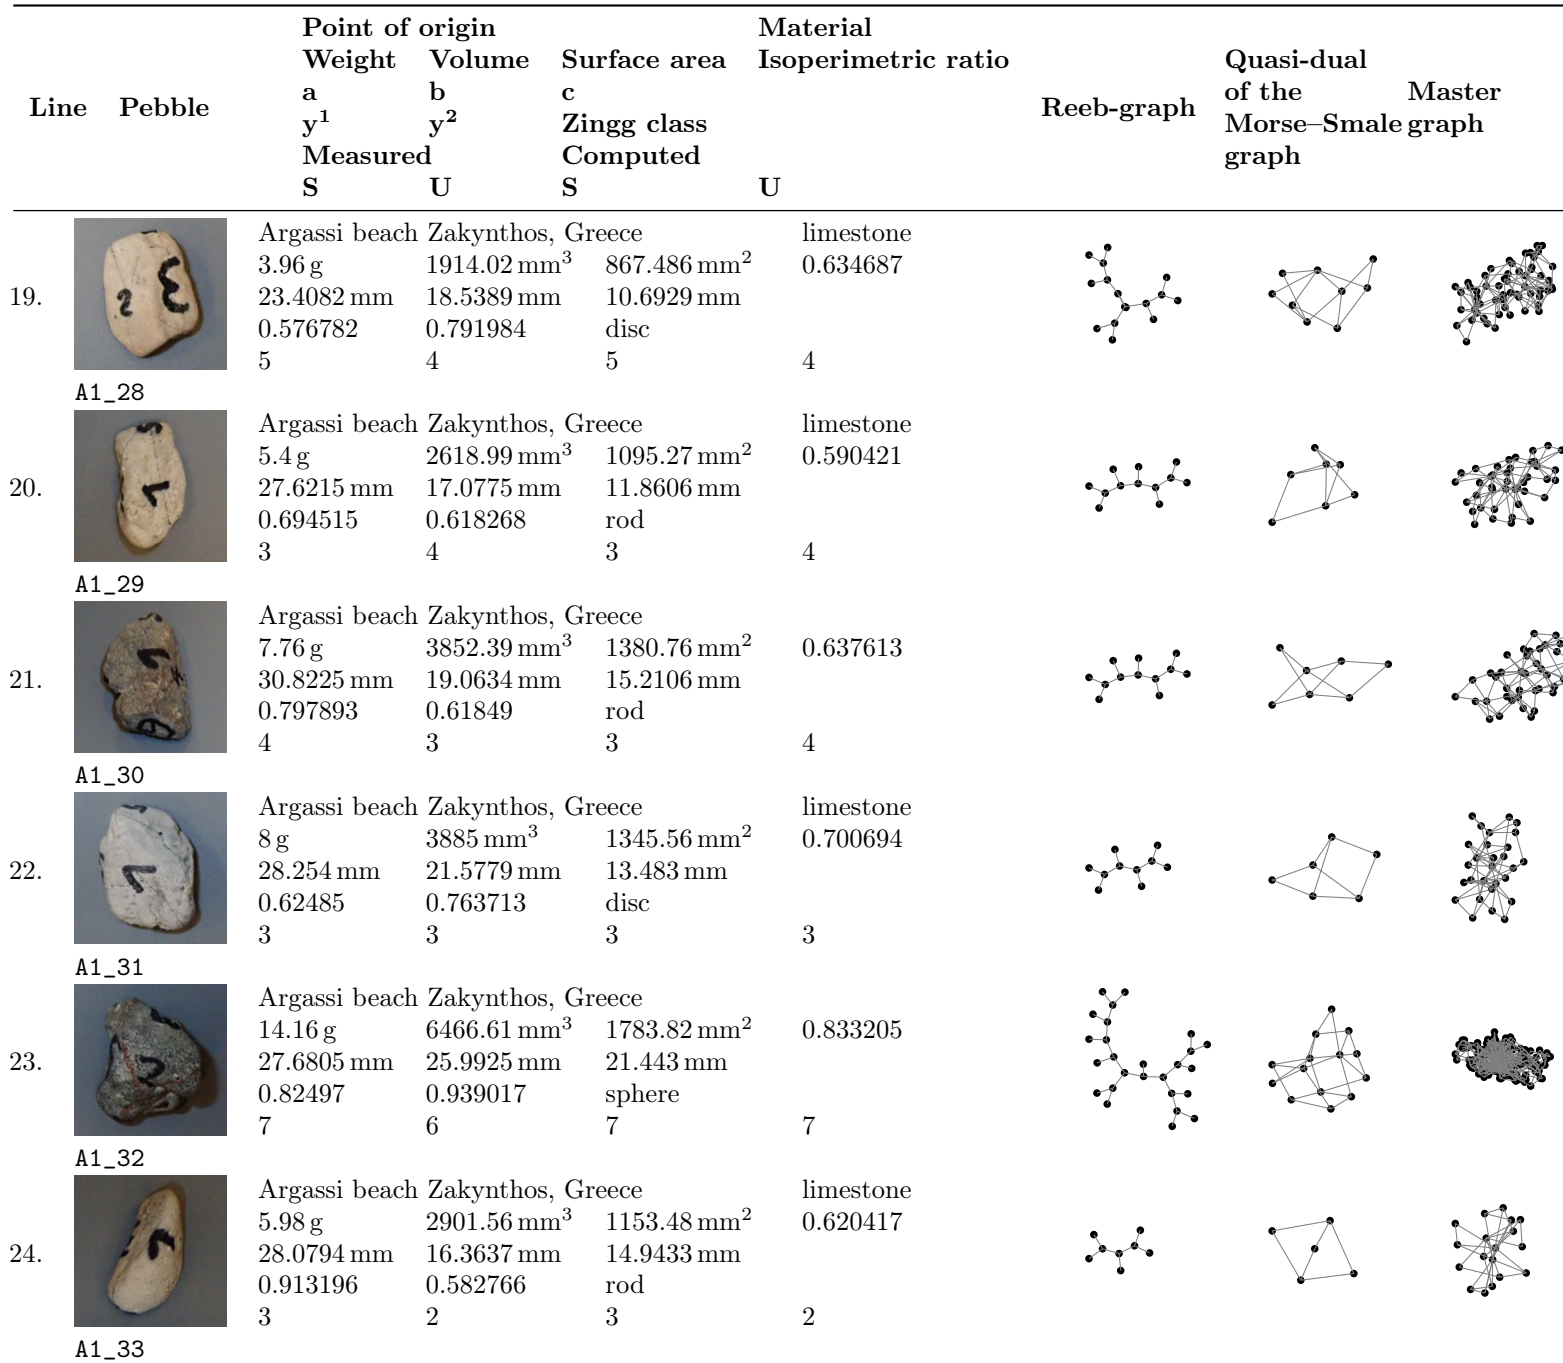  | 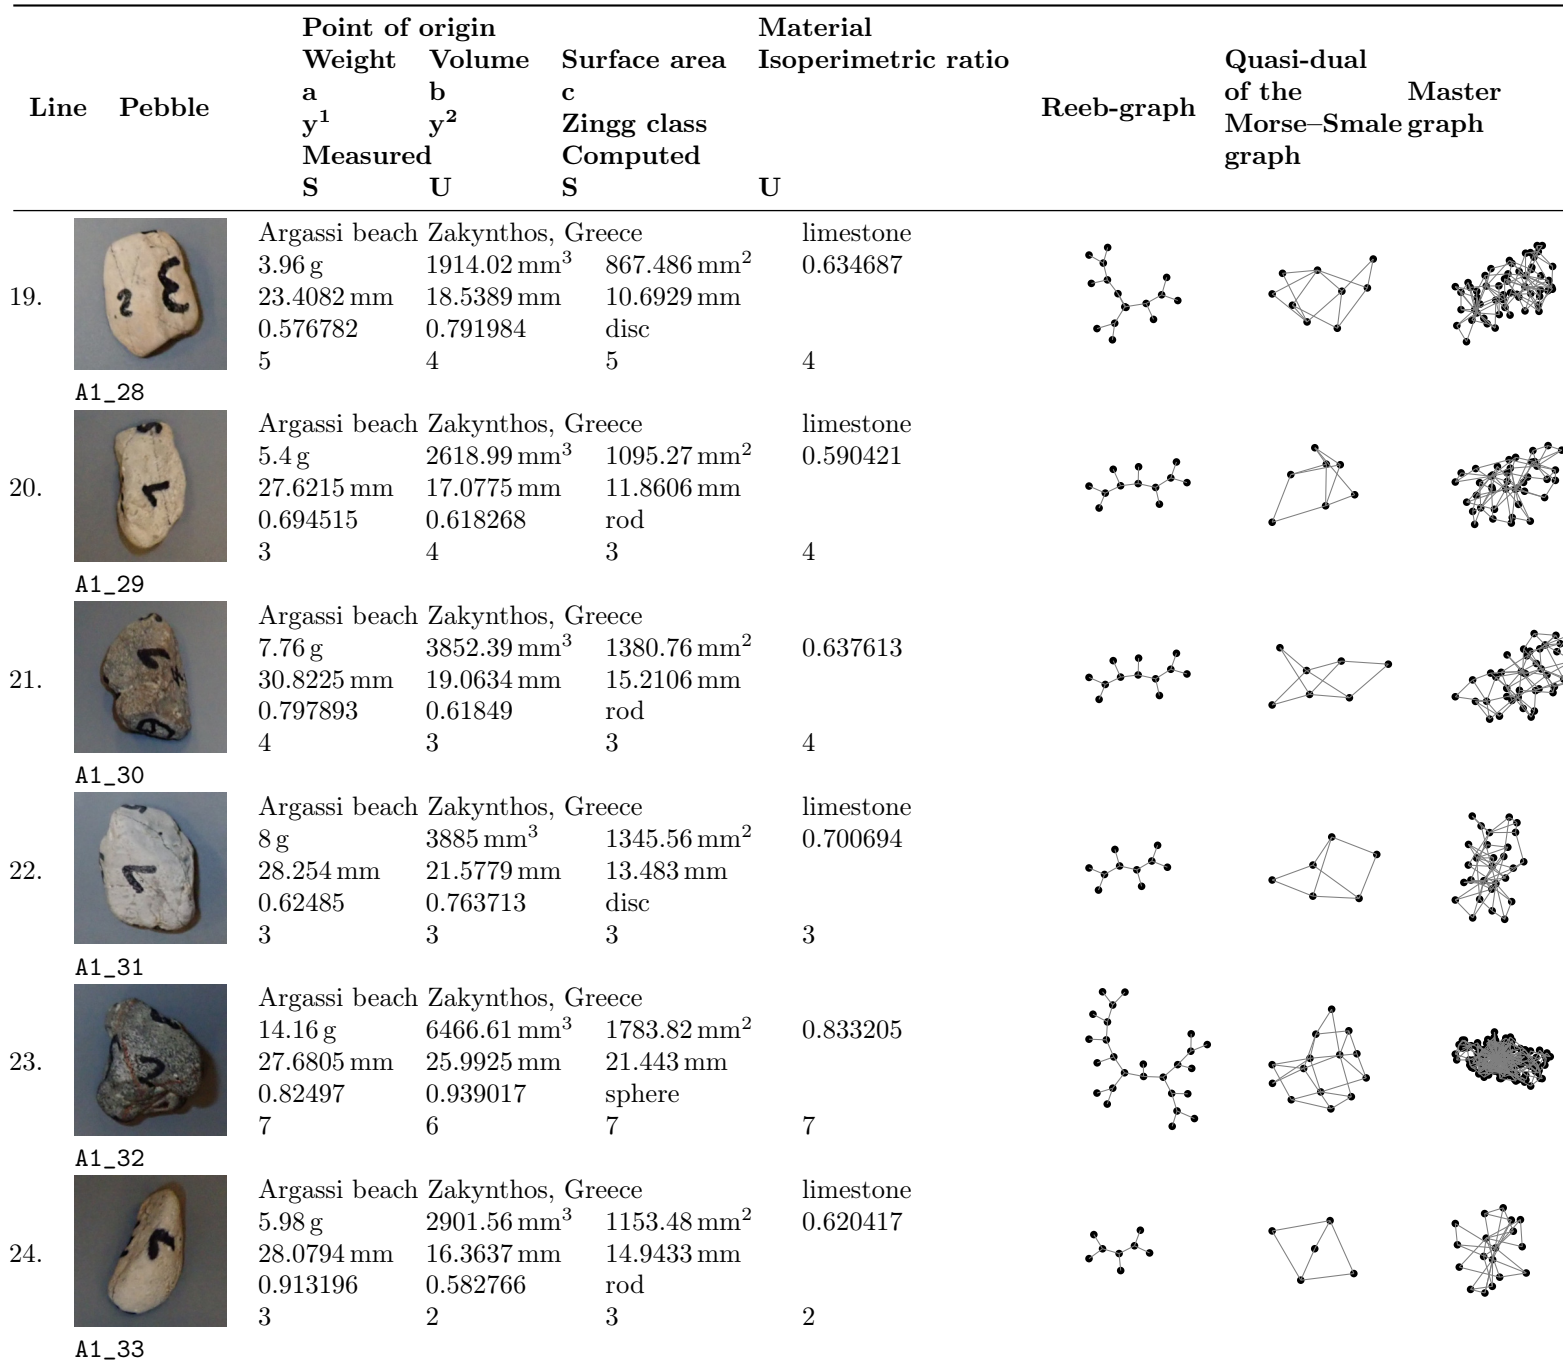  | 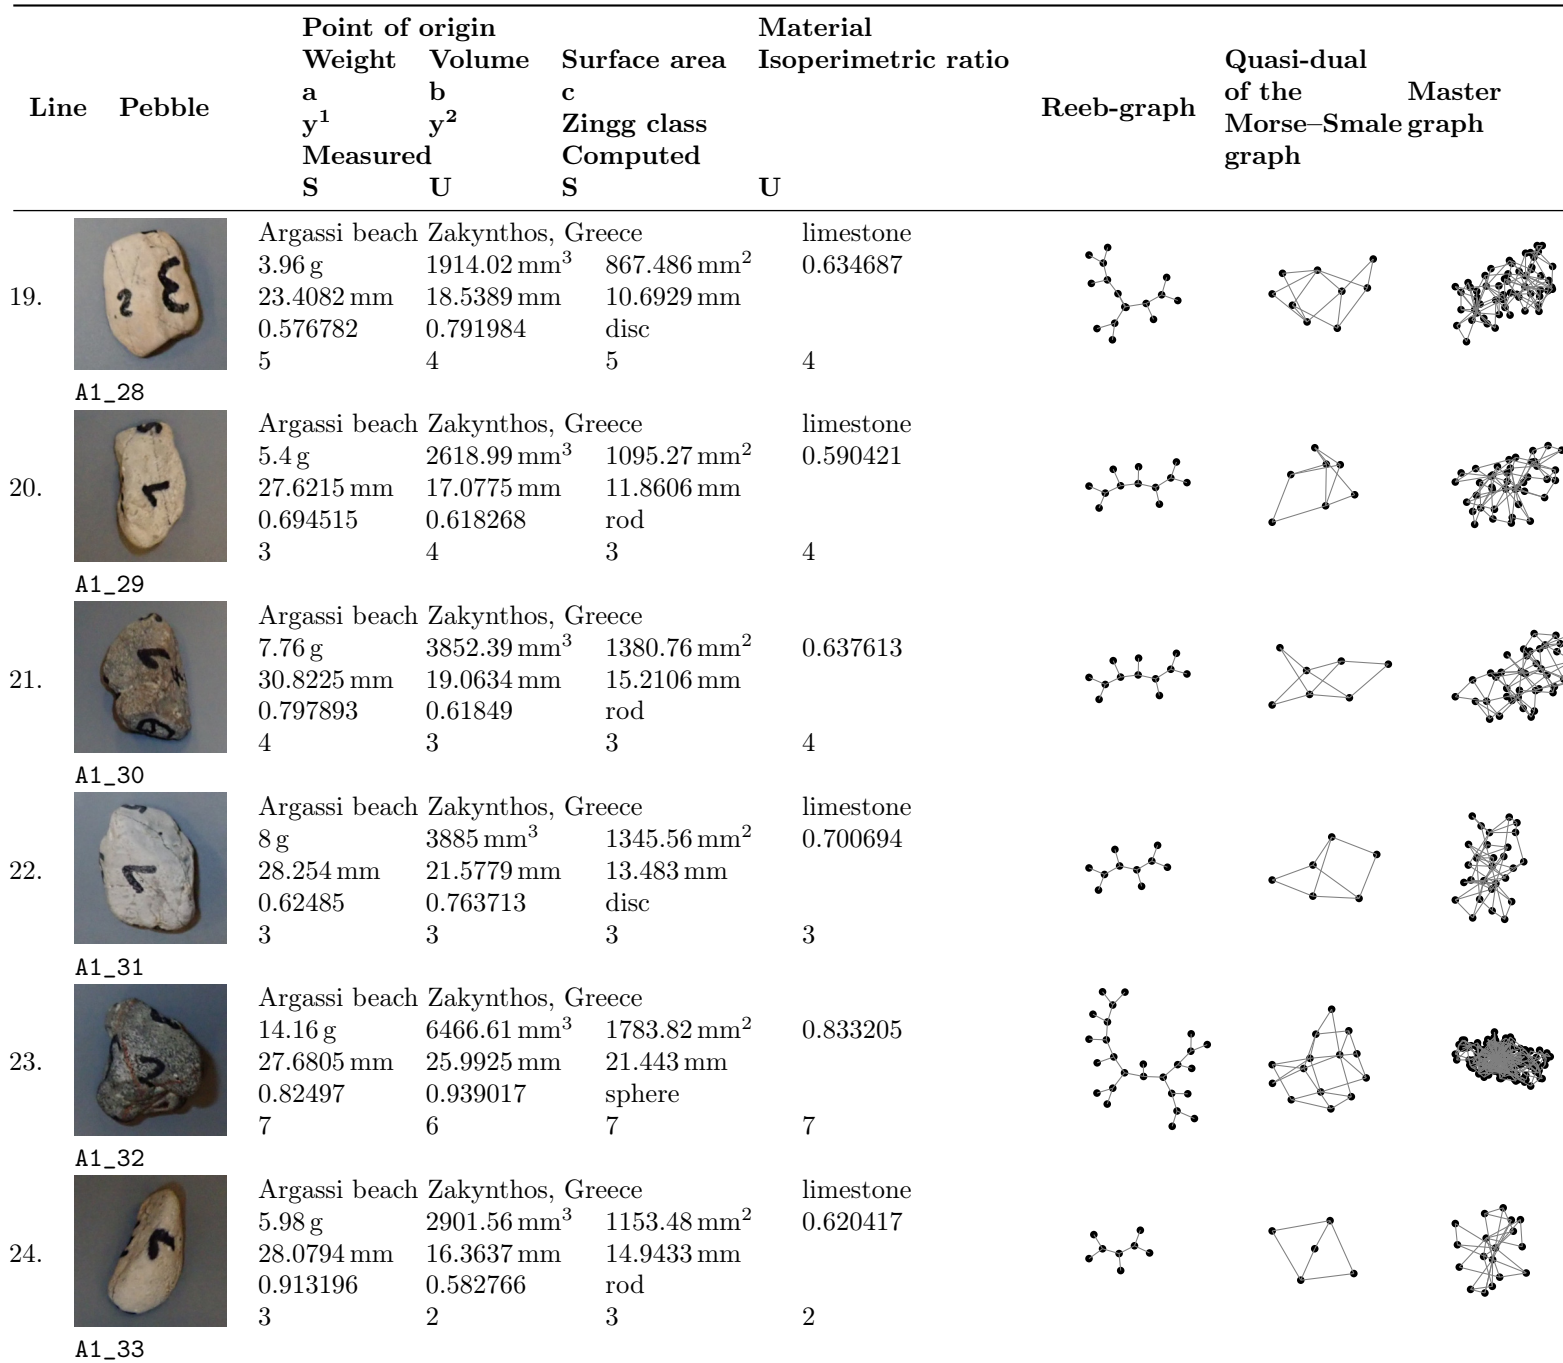  |
|      | A1_31                                                                               |                                                        |                                                                             |                                                                  |          |                                                                                       |                                                                                       |                                                                                       |
| 23.  | 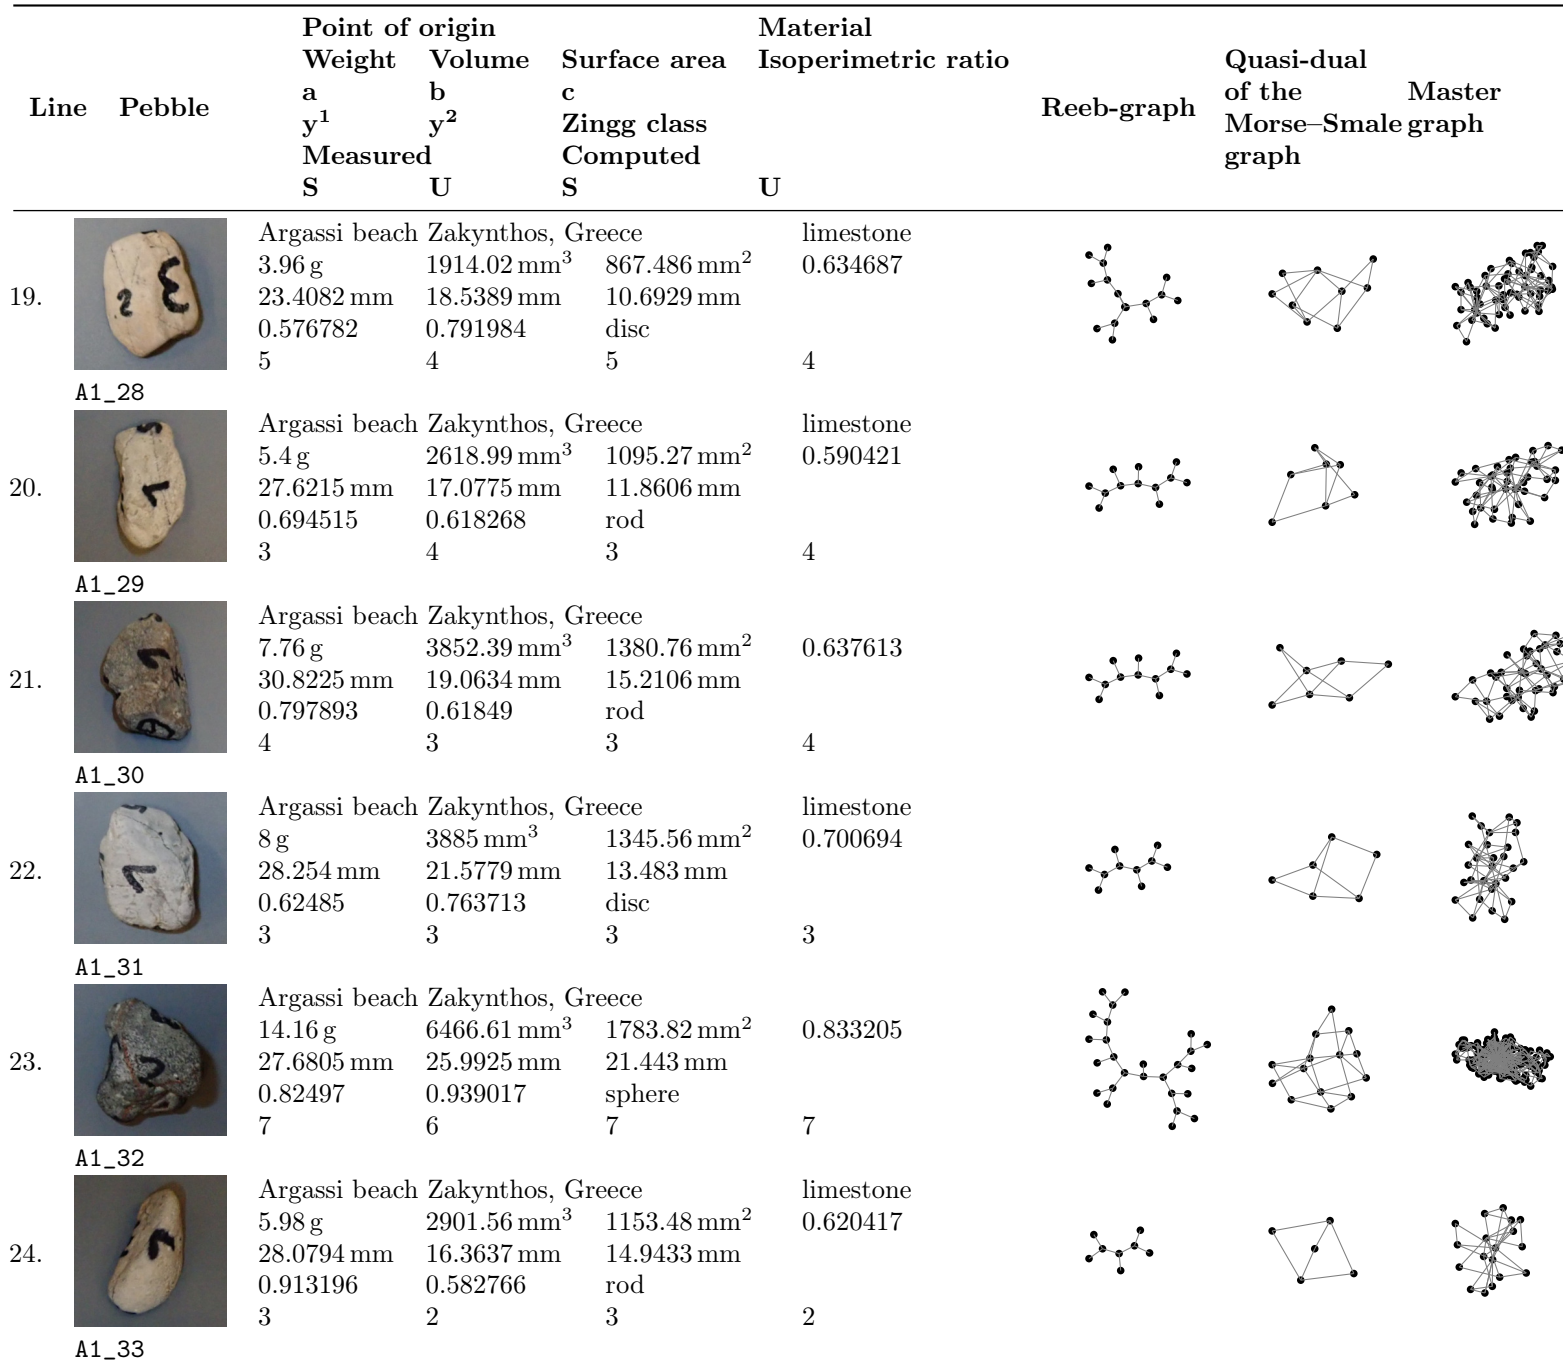 | Argassi beach<br>14.16 g<br>27.6805 mm<br>0.82497<br>7 | Zakynthos, Greece<br>6466.61 mm <sup>3</sup><br>25.9925 mm<br>0.939017<br>6 | limestone<br>1783.82 mm <sup>2</sup><br>21.443 mm<br>sphere<br>7 | 0.833205 | 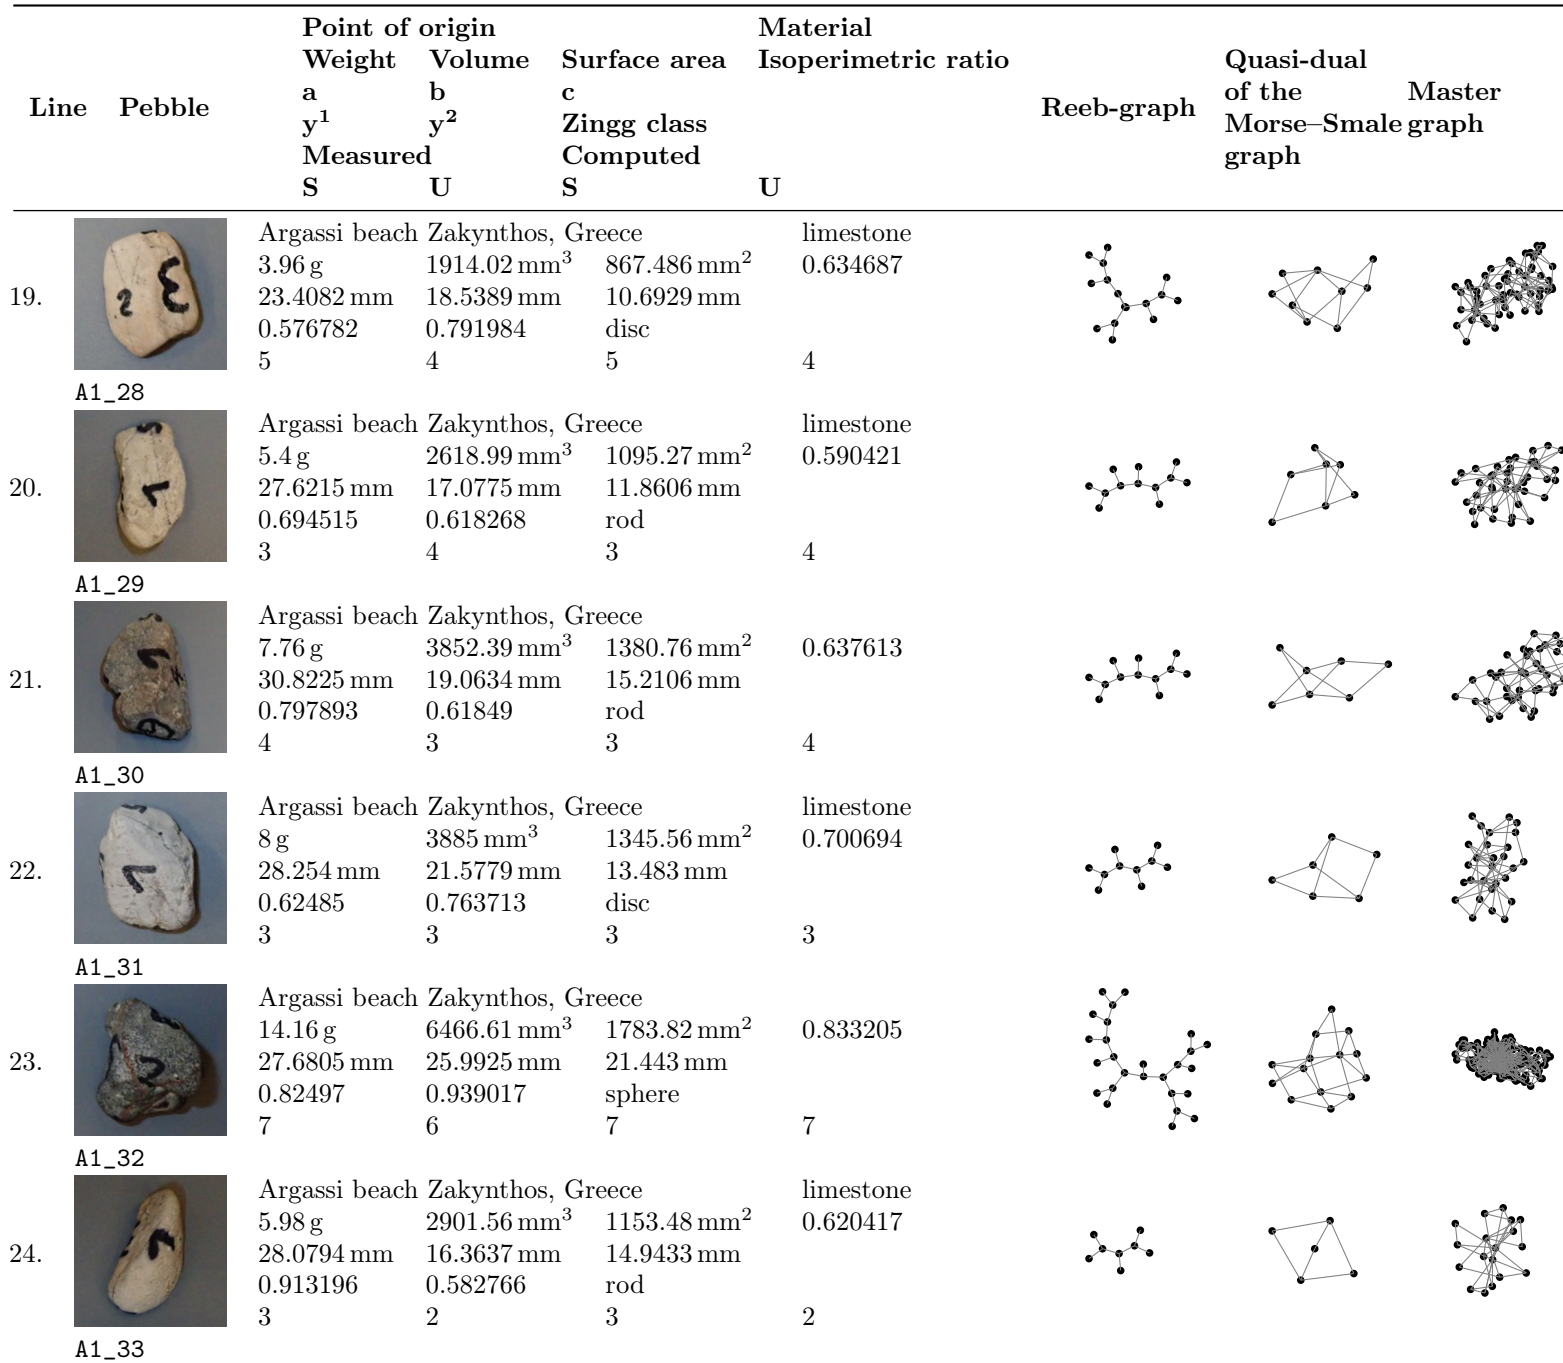 | 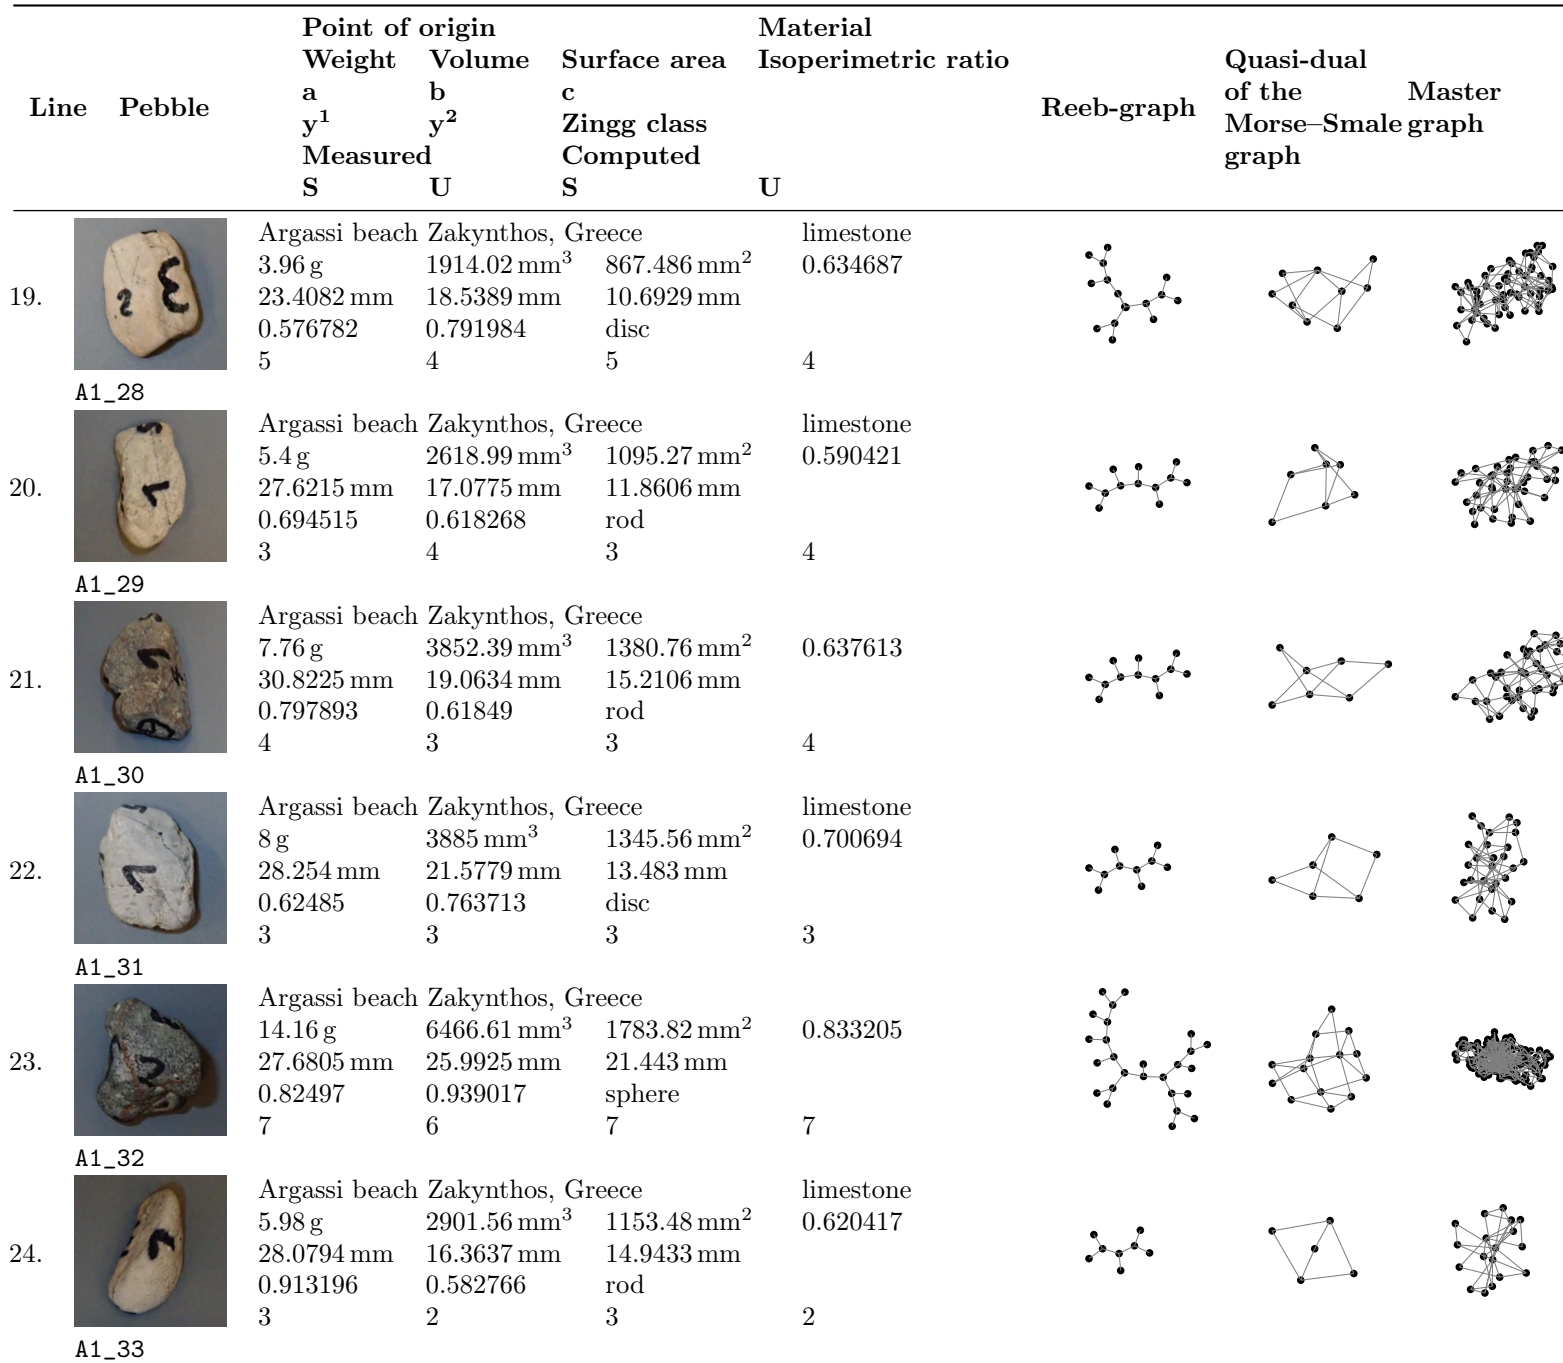 | 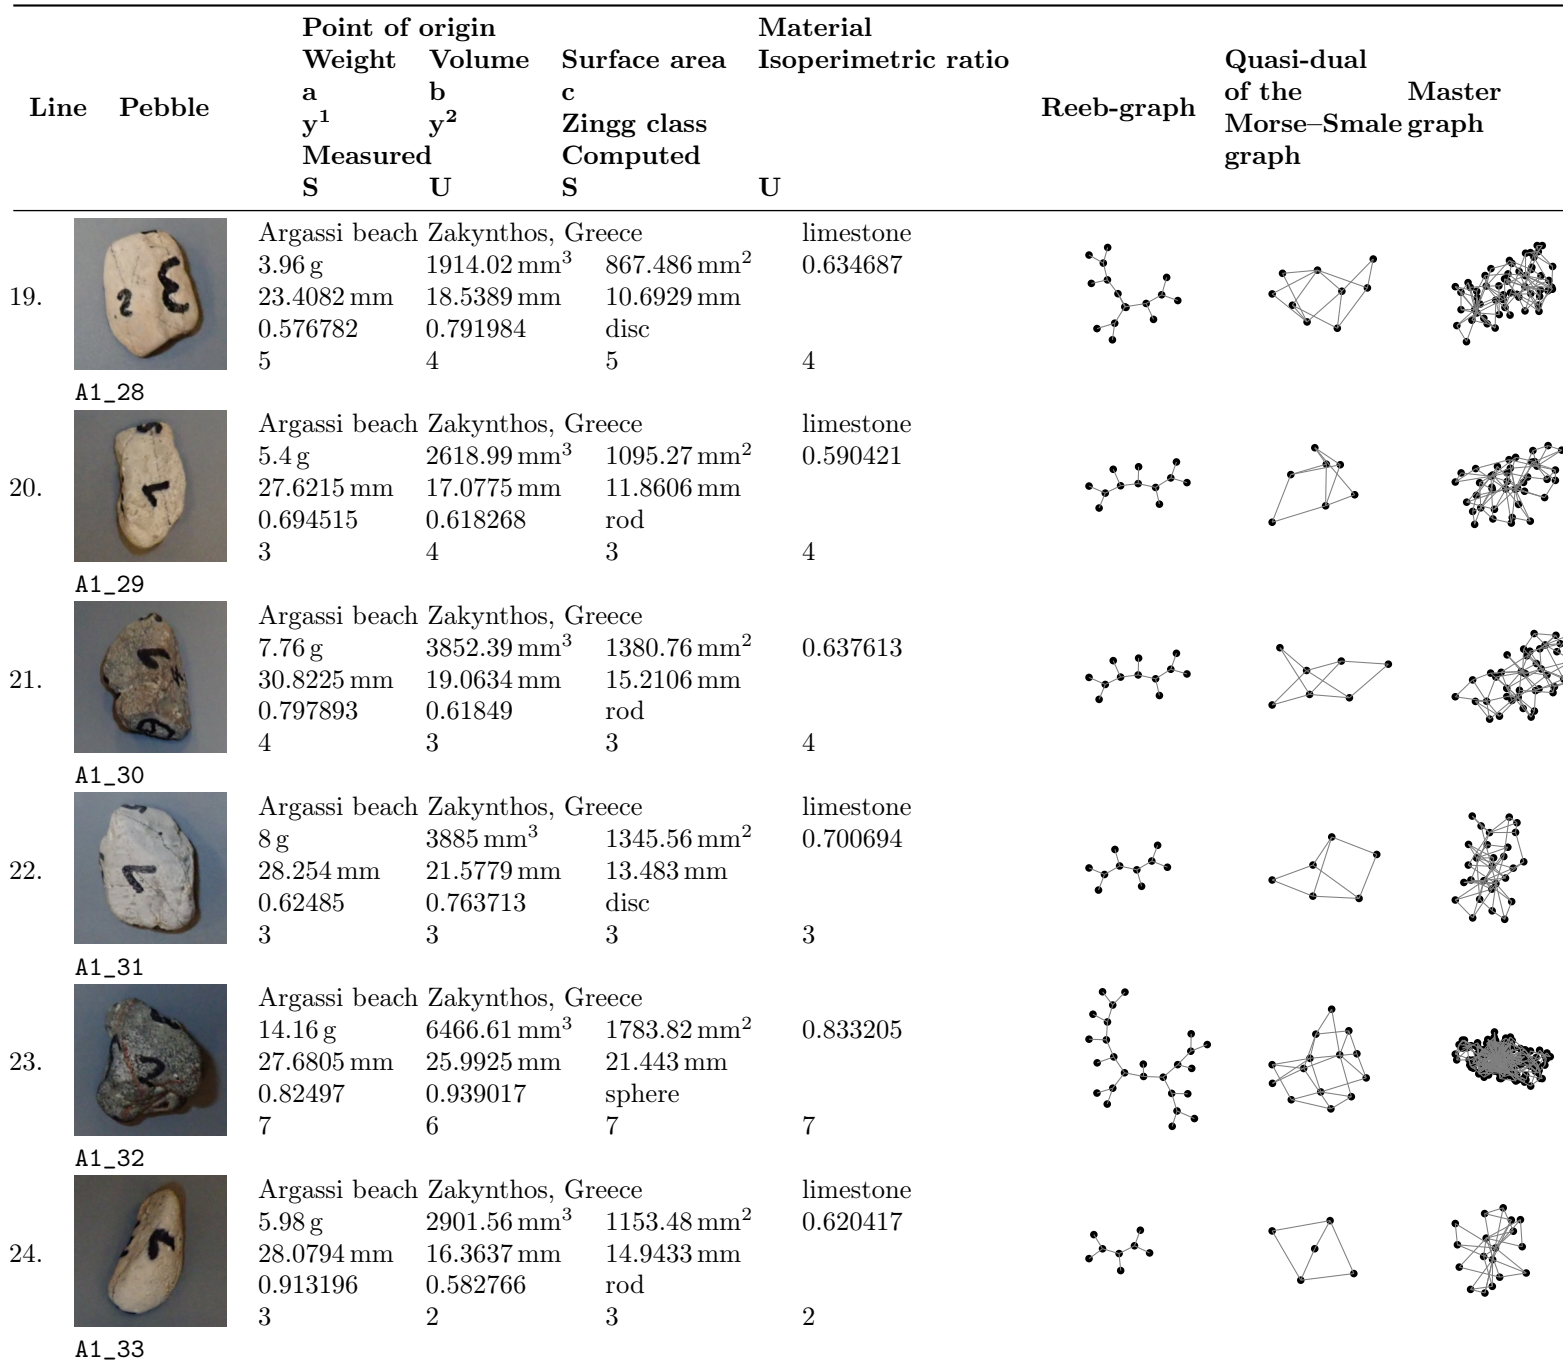 |
|      | A1_32                                                                               |                                                        |                                                                             |                                                                  |          |                                                                                       |                                                                                       |                                                                                       |
| 24.  | 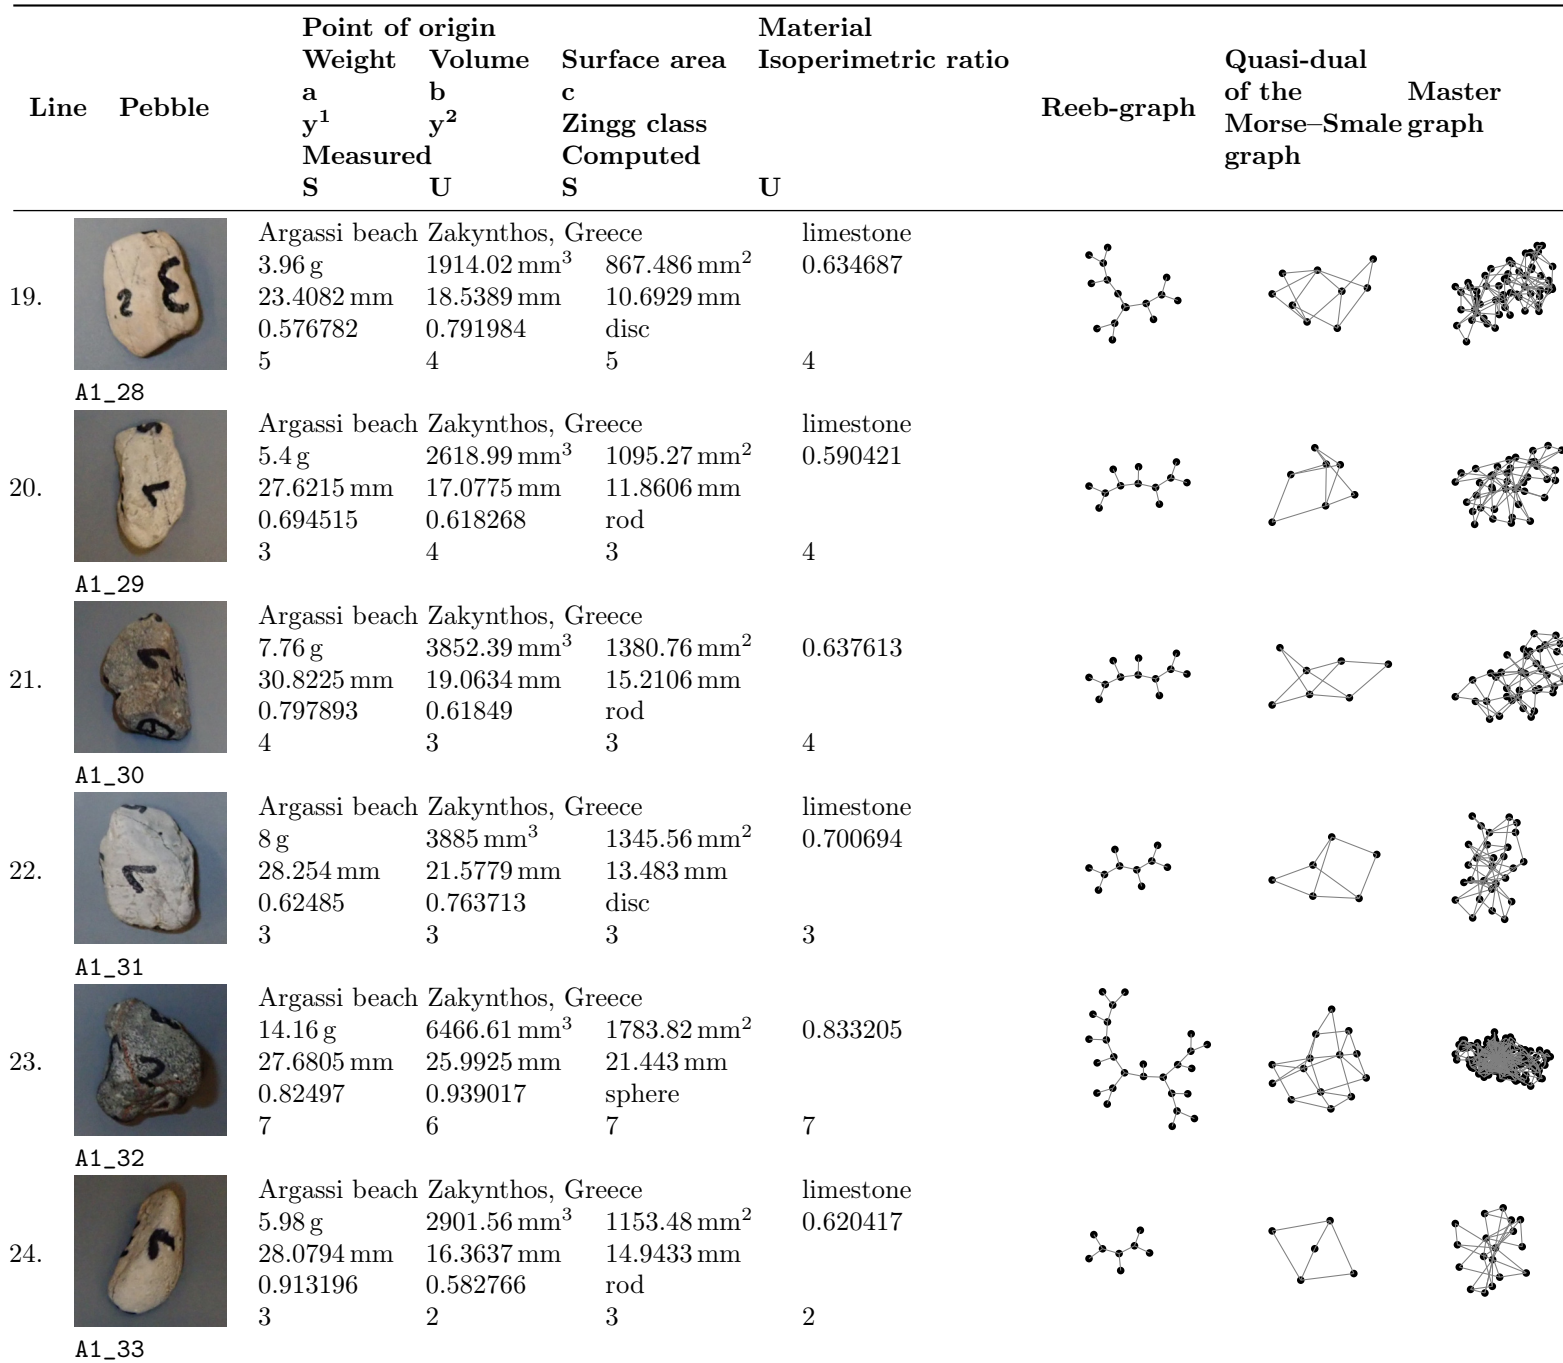 | Argassi beach<br>5.98 g<br>28.0794 mm<br>0.913196<br>3 | Zakynthos, Greece<br>2901.56 mm <sup>3</sup><br>16.3637 mm<br>0.582766<br>2 | limestone<br>1153.48 mm <sup>2</sup><br>14.9433 mm<br>rod<br>3   | 0.620417 | 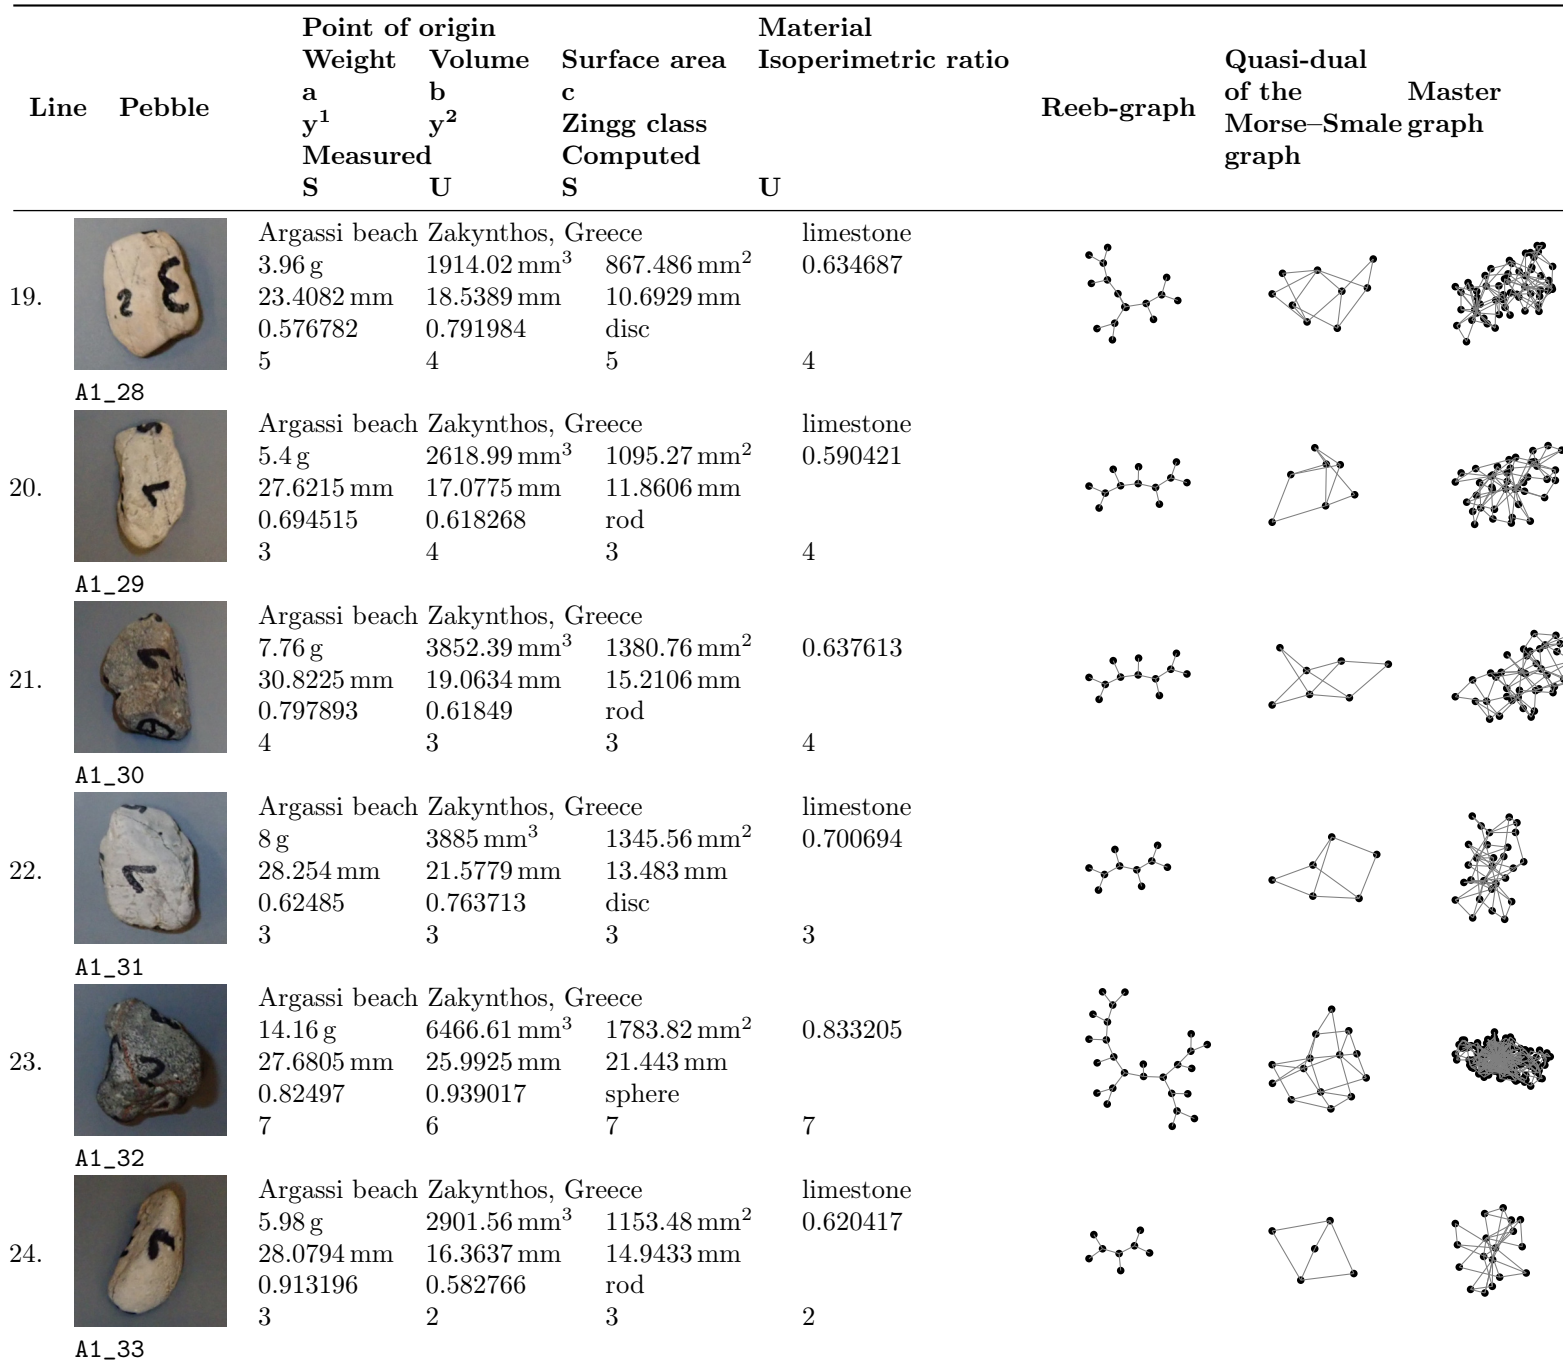 | 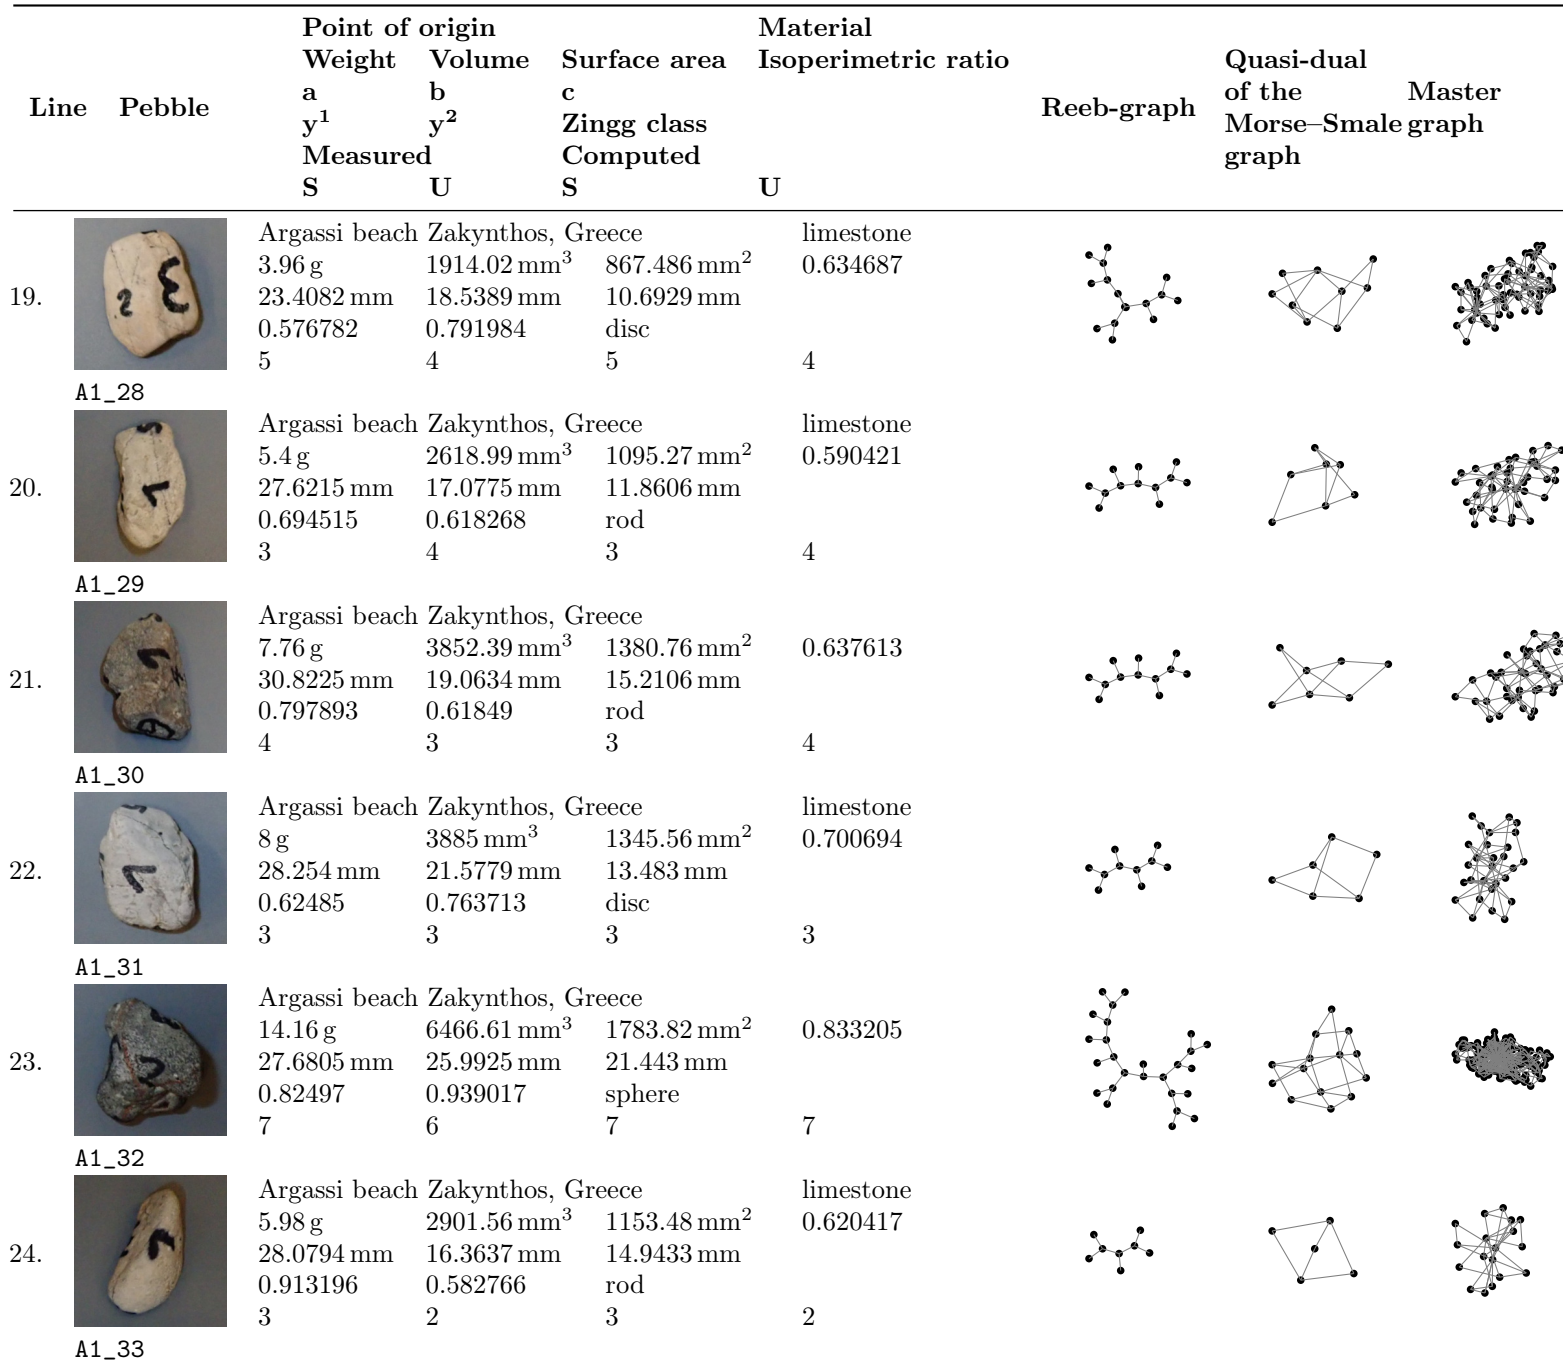 | 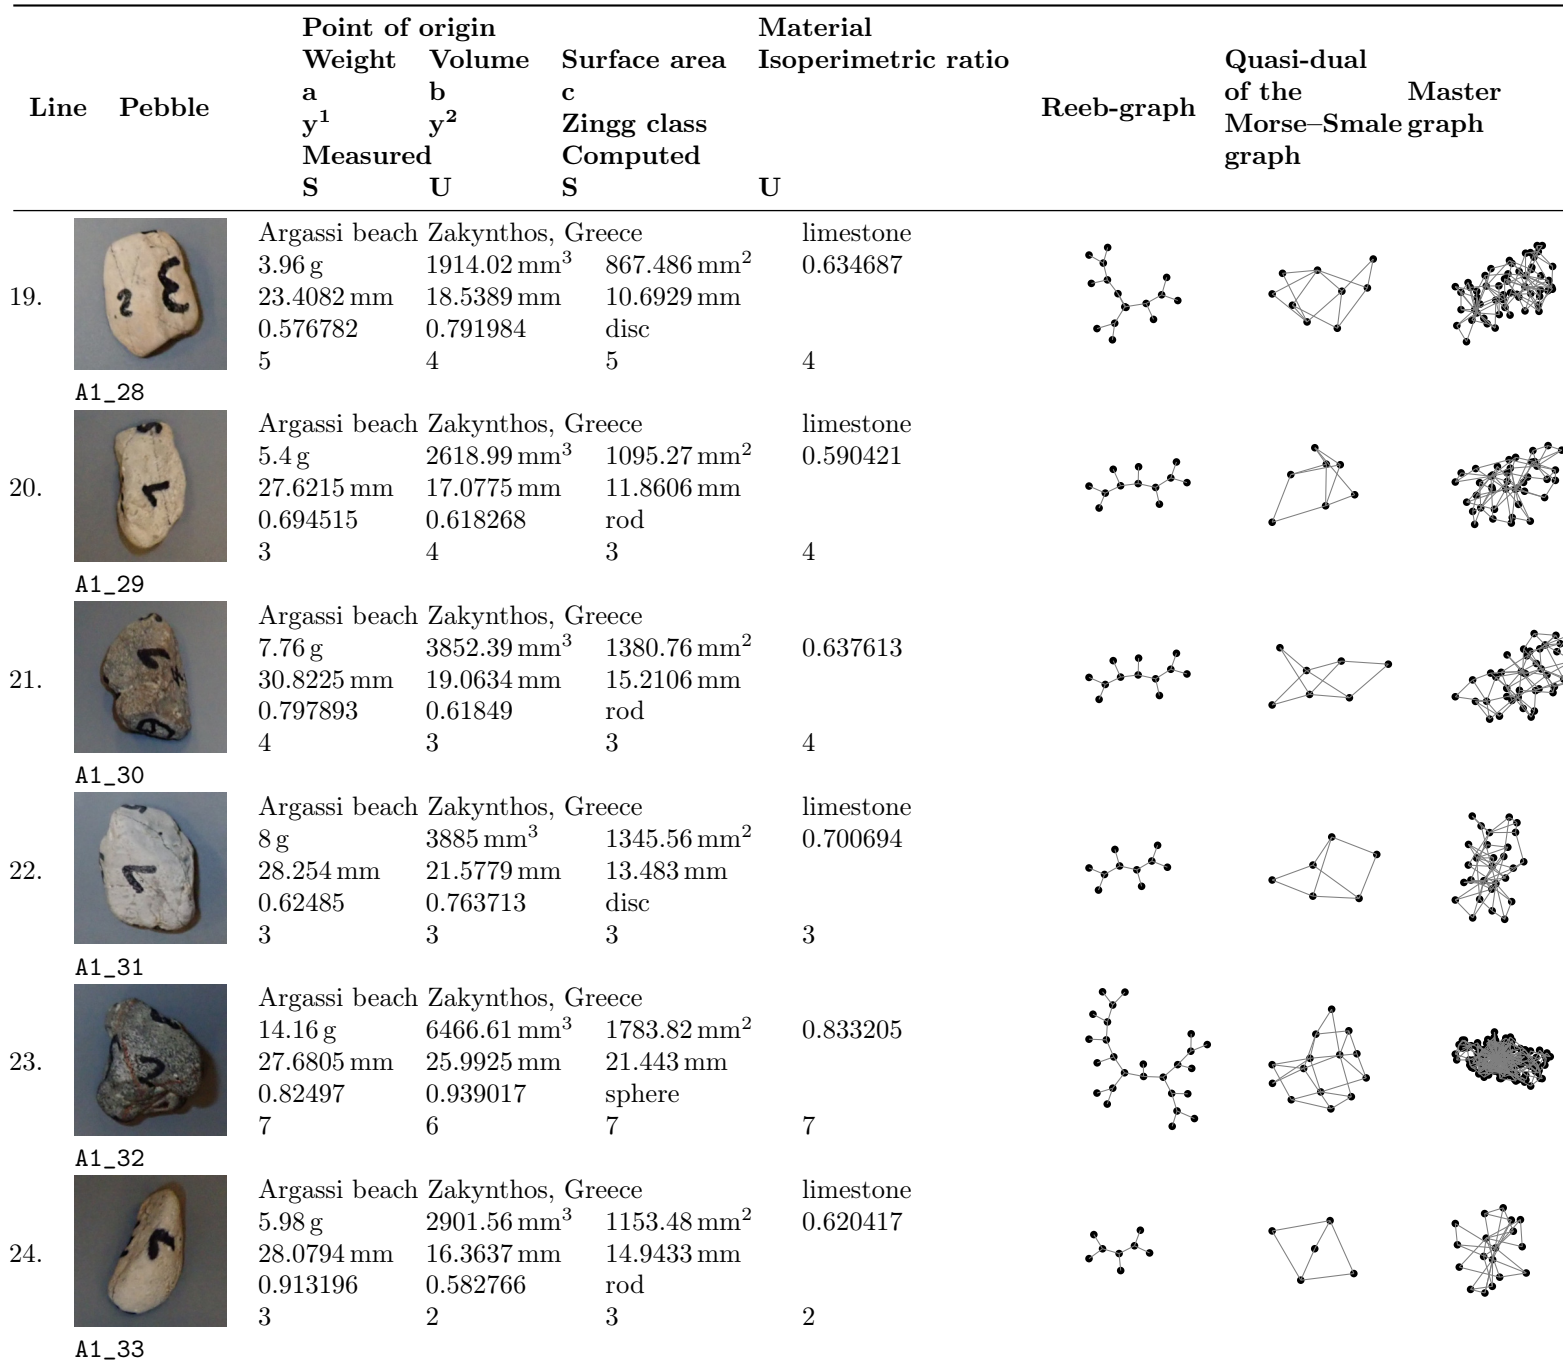 |
|      | A1_33                                                                               |                                                        |                                                                             |                                                                  |          |                                                                                       |                                                                                       |                                                                                       |

| Line | Pebble                                                                              | Point of origin                                         |                                                                             |                                                                   | Material | Reeb-graph                                                                            | Quasi-dual<br>of the<br>Morse–Smale<br>graph                                          | Master<br>graph                                                                       |
|------|-------------------------------------------------------------------------------------|---------------------------------------------------------|-----------------------------------------------------------------------------|-------------------------------------------------------------------|----------|---------------------------------------------------------------------------------------|---------------------------------------------------------------------------------------|---------------------------------------------------------------------------------------|
|      |                                                                                     | Weight                                                  | Volume                                                                      | Surface area                                                      |          |                                                                                       |                                                                                       |                                                                                       |
|      |                                                                                     | a                                                       | b                                                                           | c                                                                 |          |                                                                                       |                                                                                       |                                                                                       |
|      |                                                                                     | y <sup>1</sup><br>Measured<br>S                         | y <sup>2</sup><br>U                                                         | Zingg class<br>Computed<br>S                                      |          |                                                                                       |                                                                                       |                                                                                       |
| 25.  | 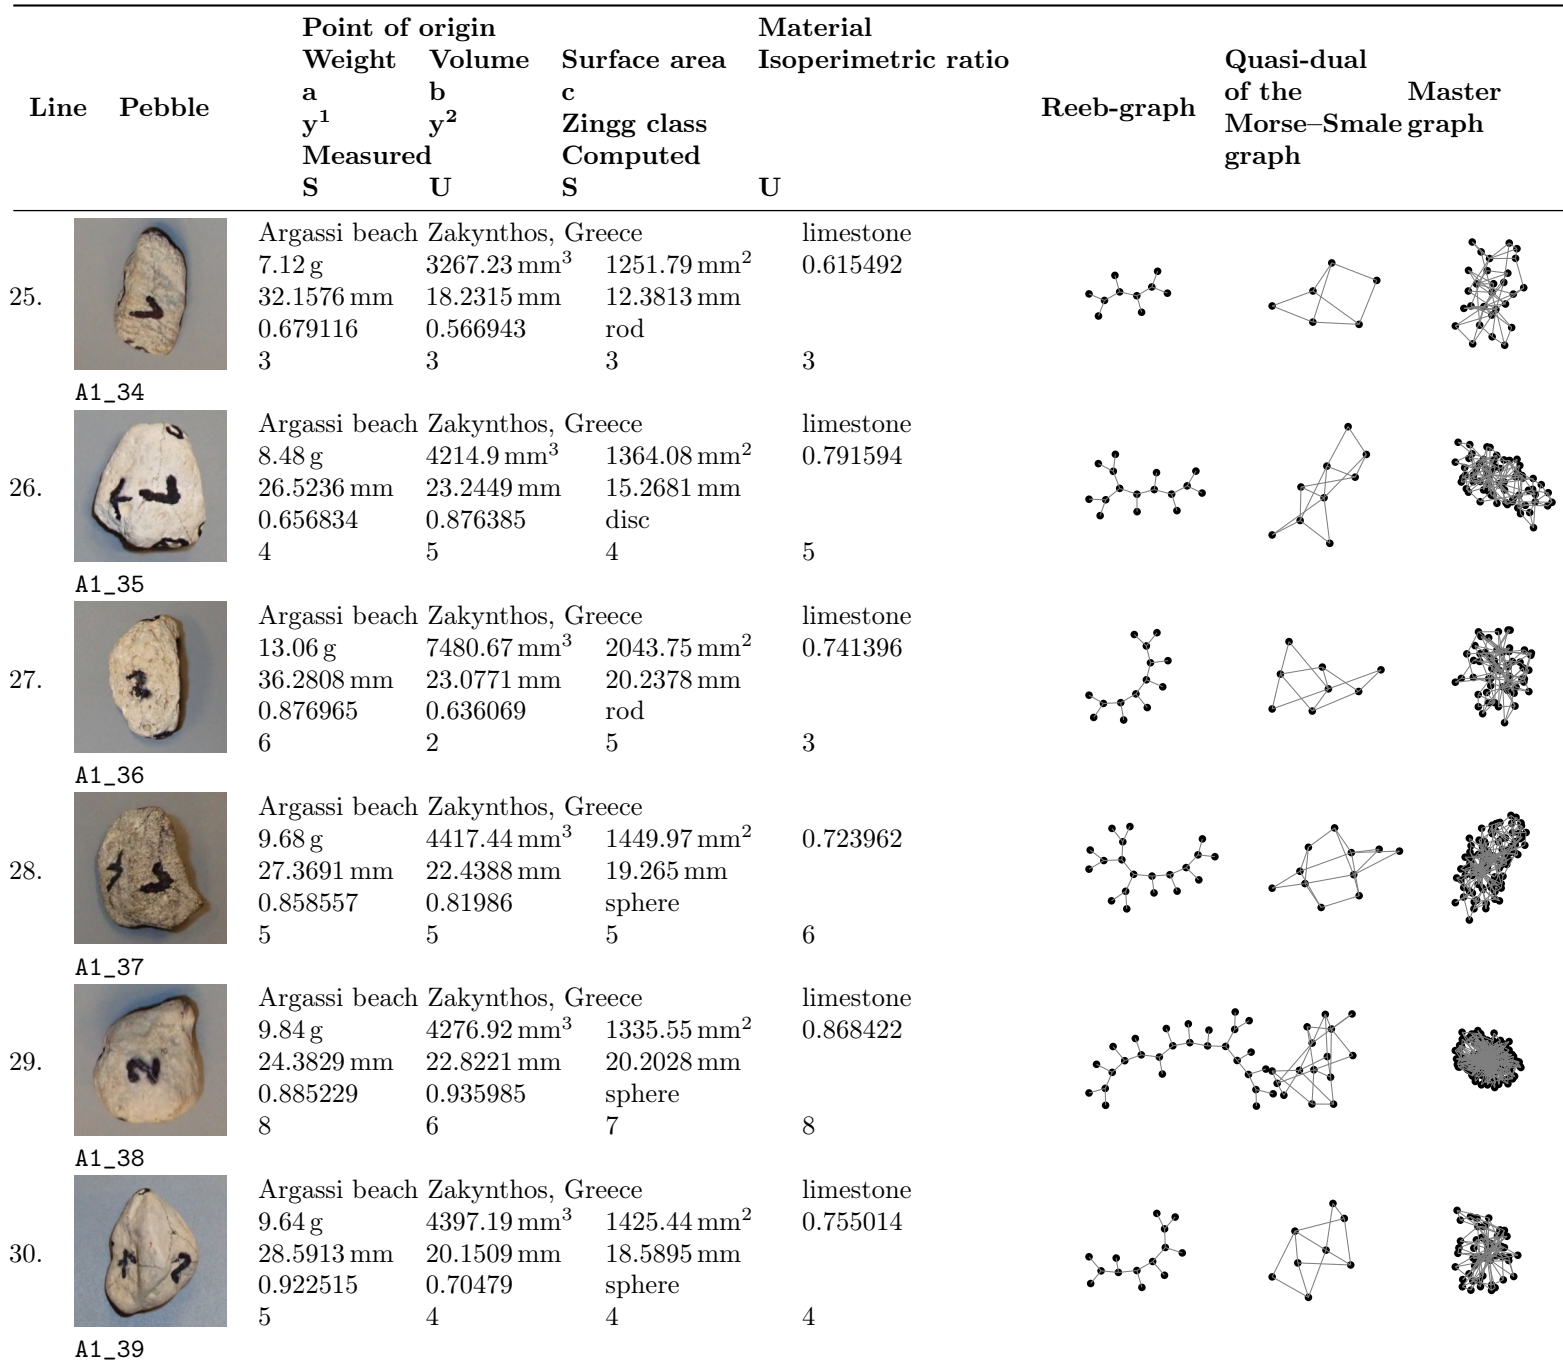   | Argassi beach<br>7.12 g<br>32.1576 mm<br>0.679116<br>3  | Zakynthos, Greece<br>3267.23 mm <sup>3</sup><br>18.2315 mm<br>0.566943<br>3 | limestone<br>1251.79 mm <sup>2</sup><br>12.3813 mm<br>rod<br>3    | 0.615492 | 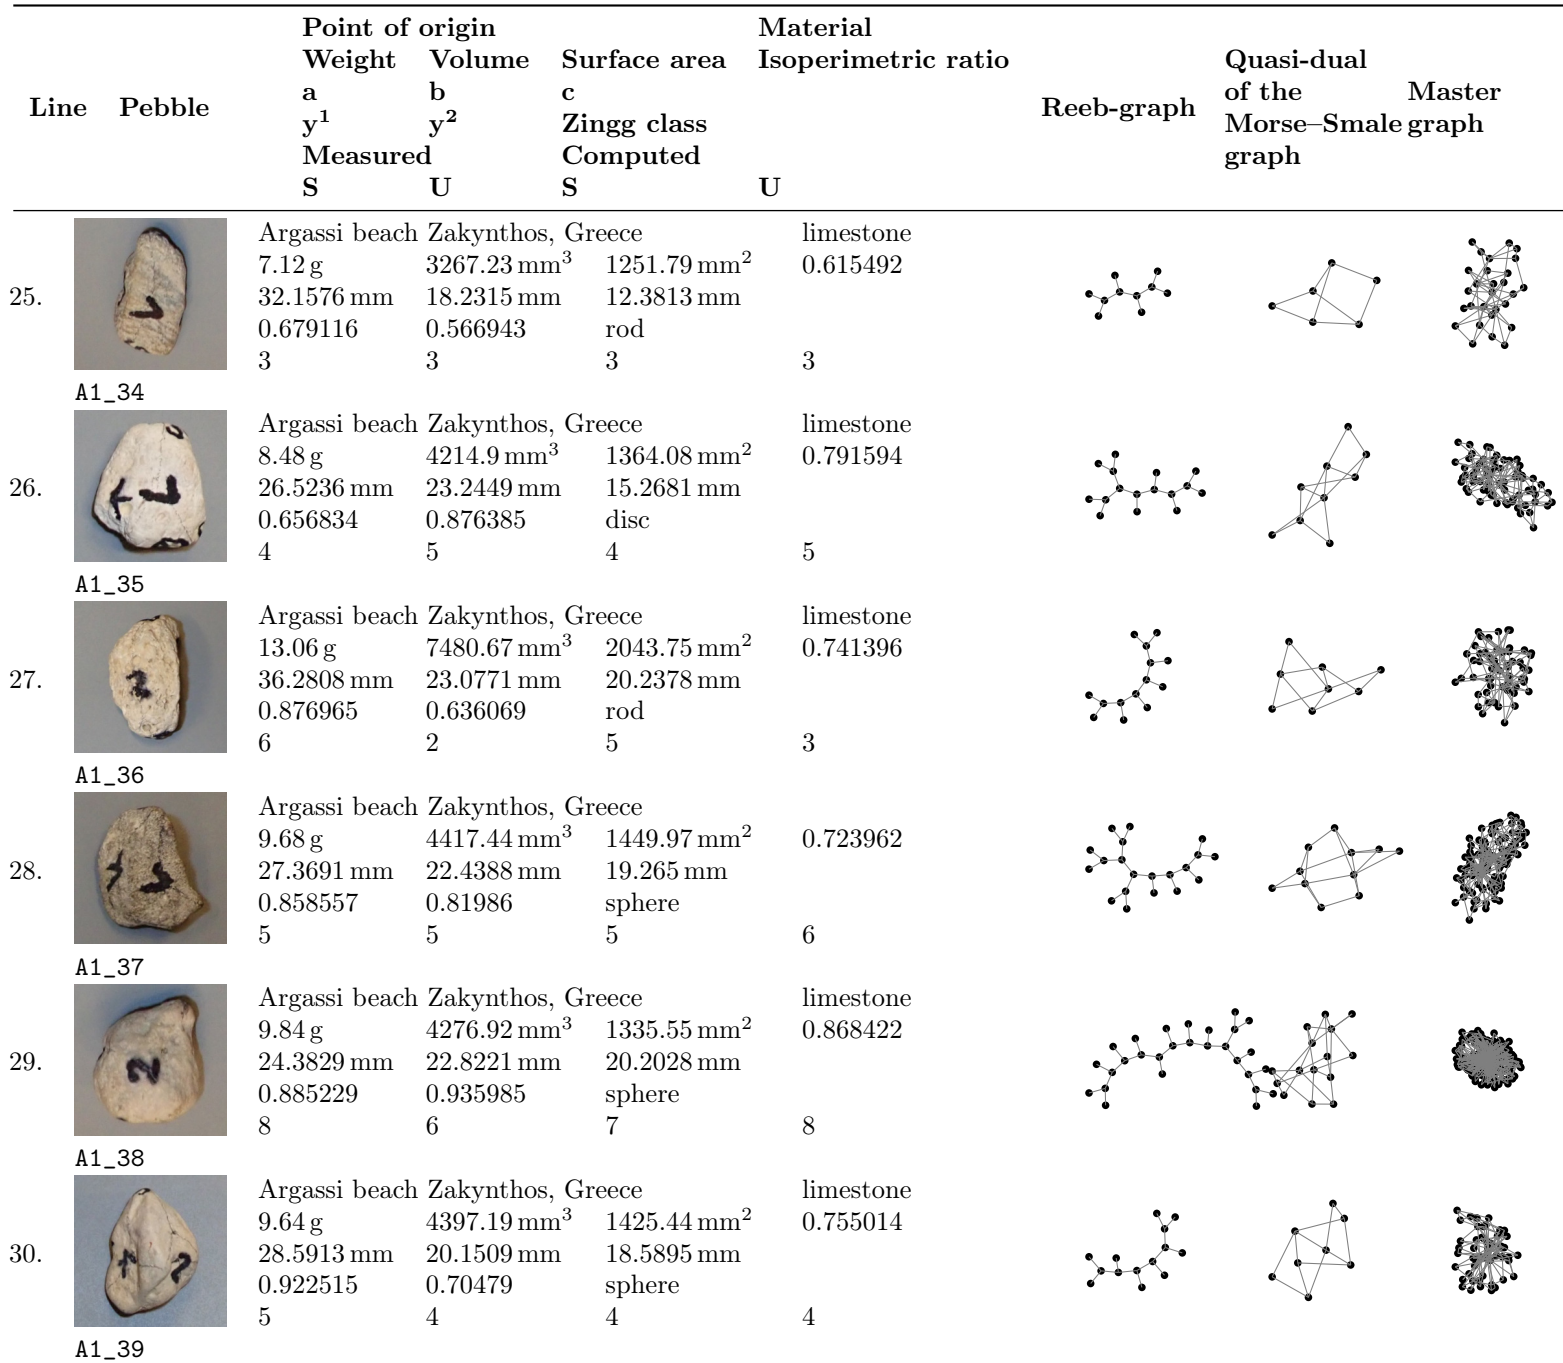   | 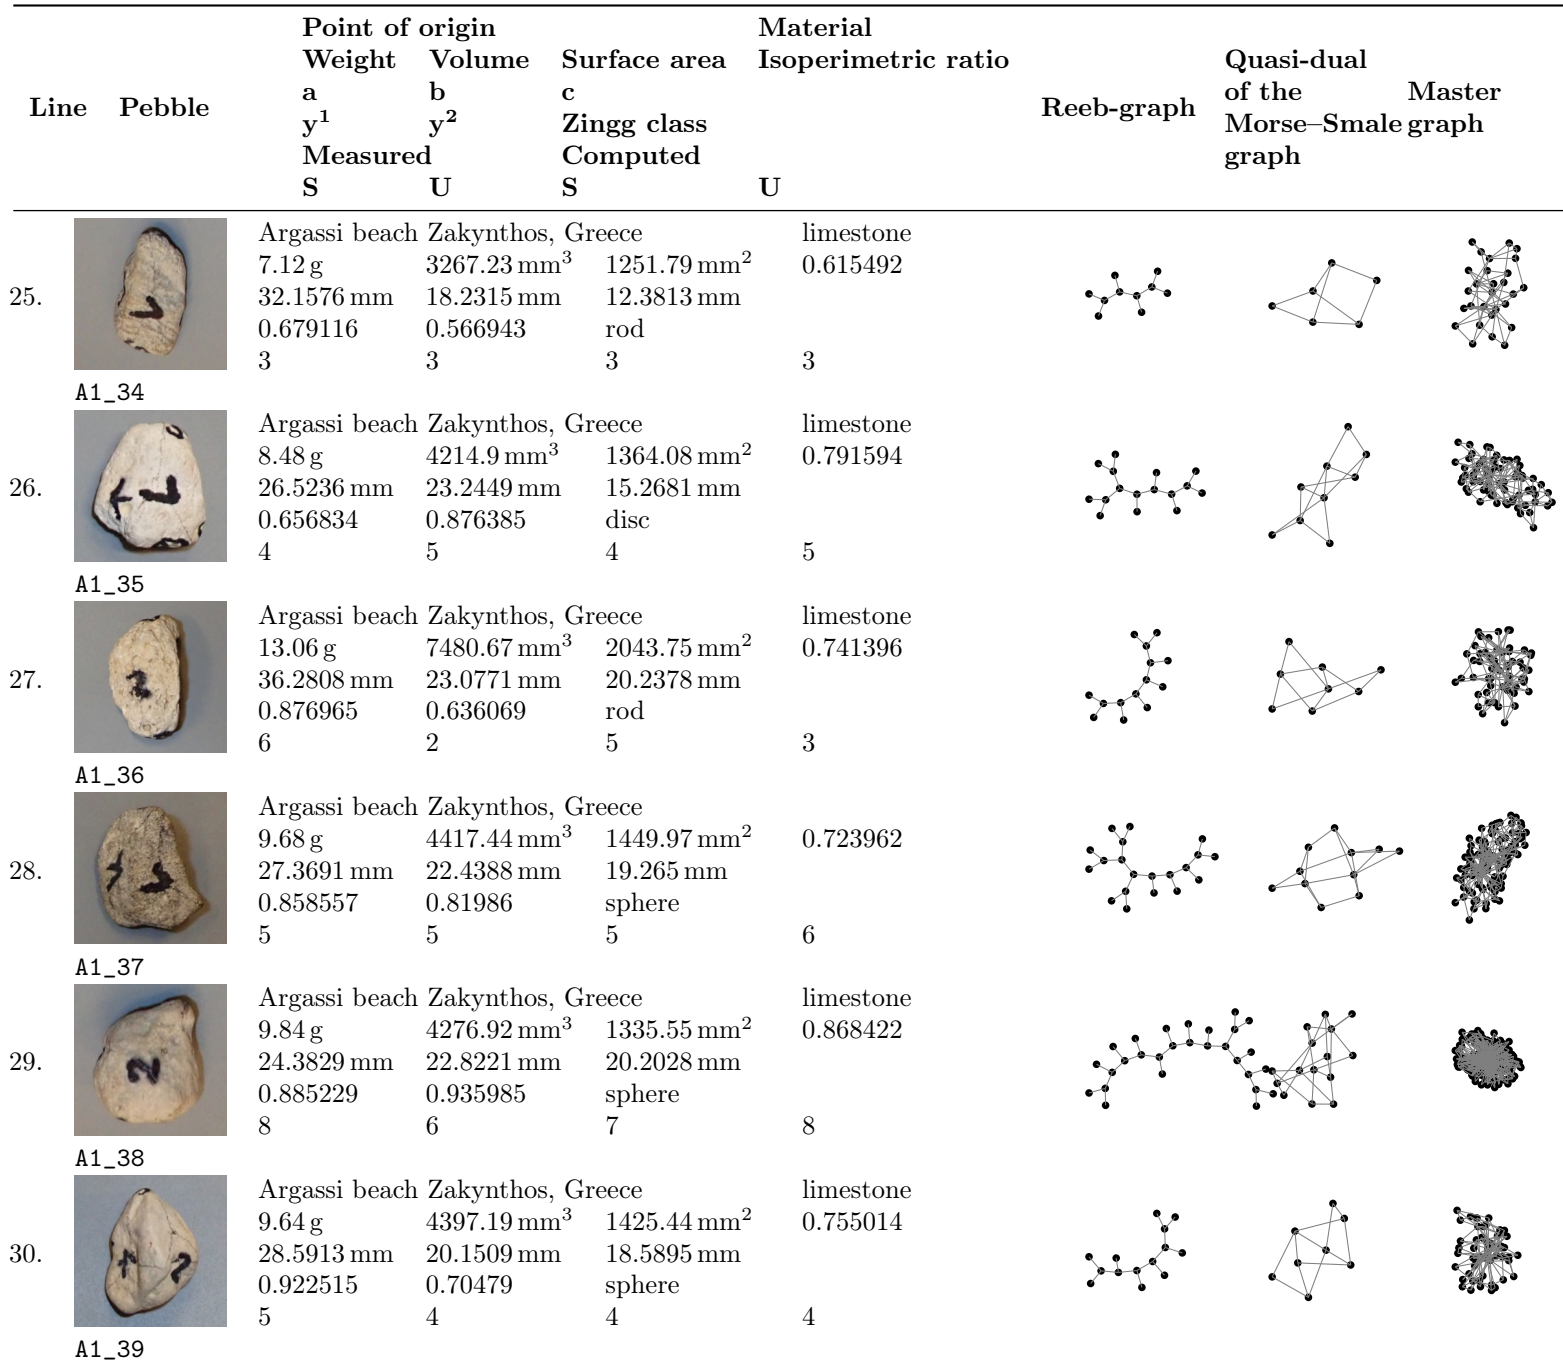   | 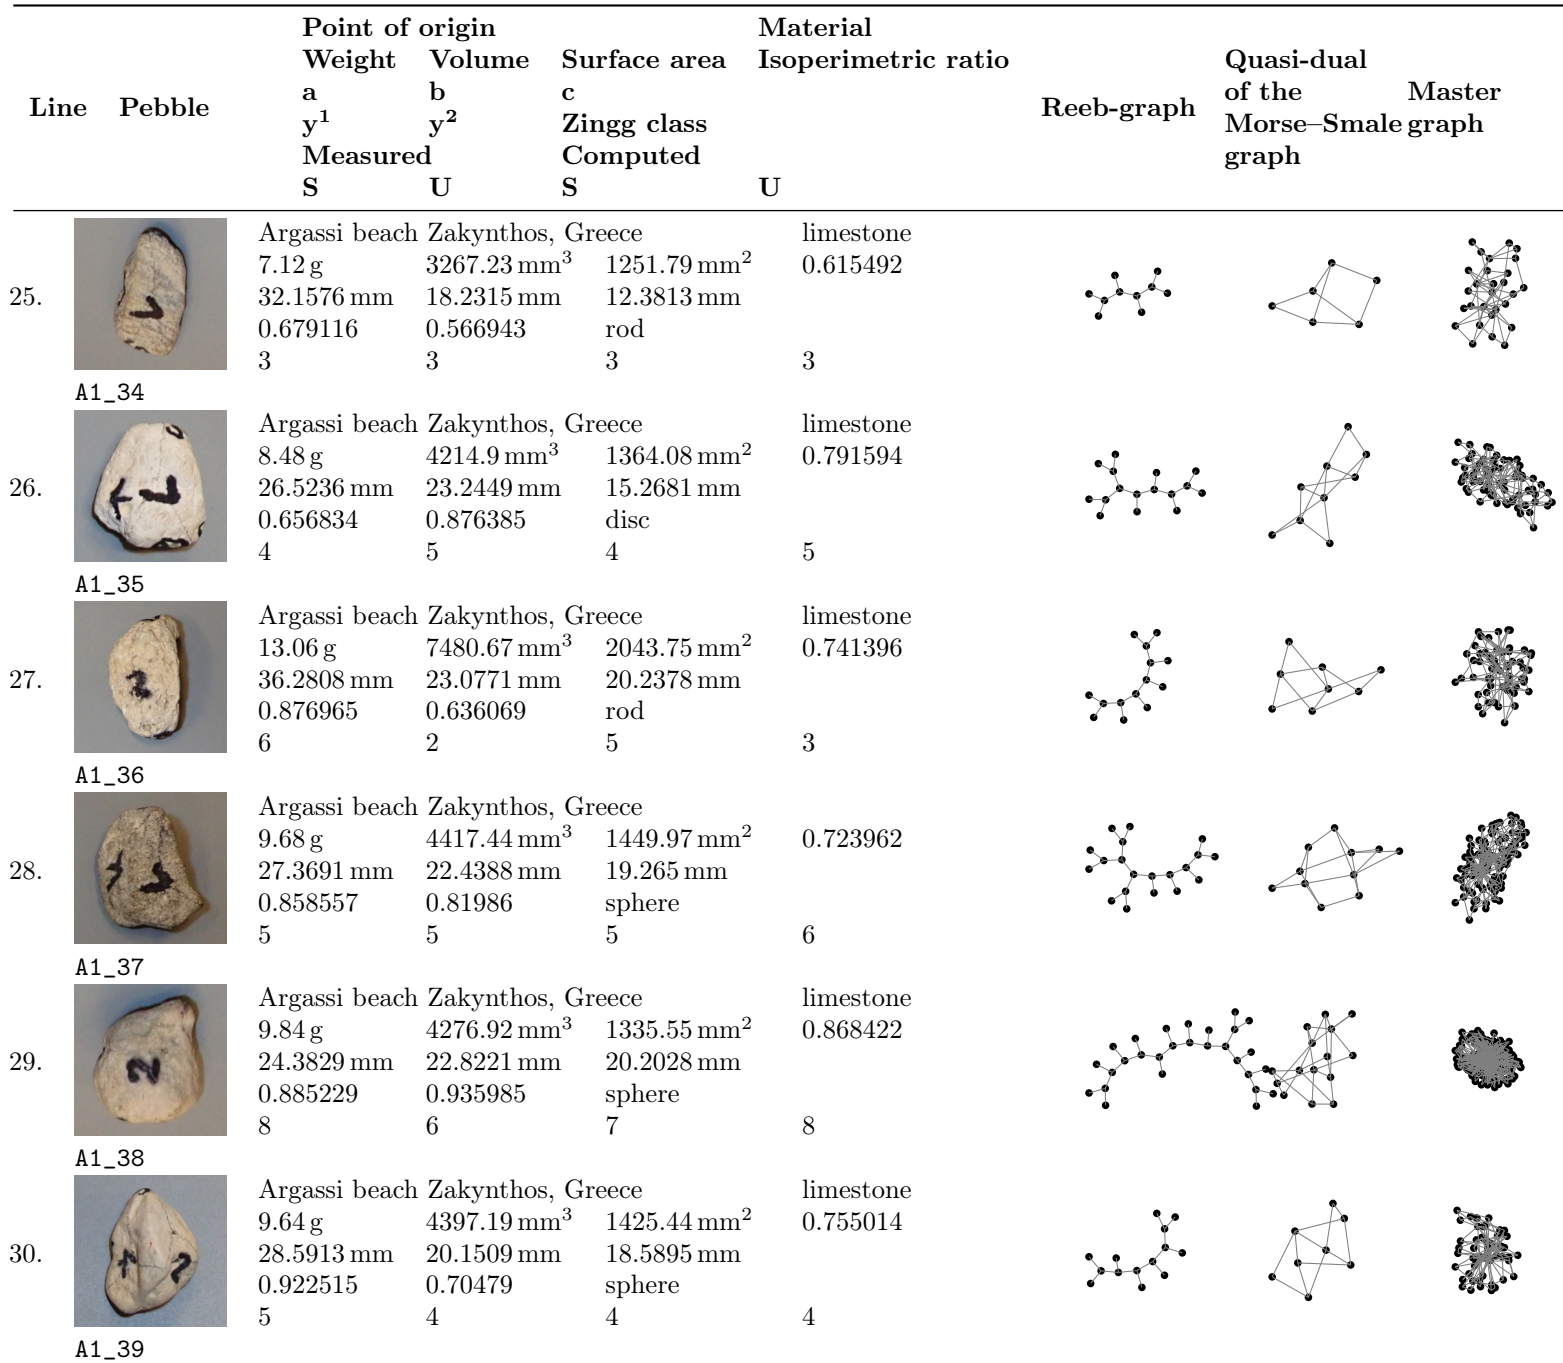   |
|      | A1_34                                                                               |                                                         |                                                                             |                                                                   |          |                                                                                       |                                                                                       |                                                                                       |
| 26.  | 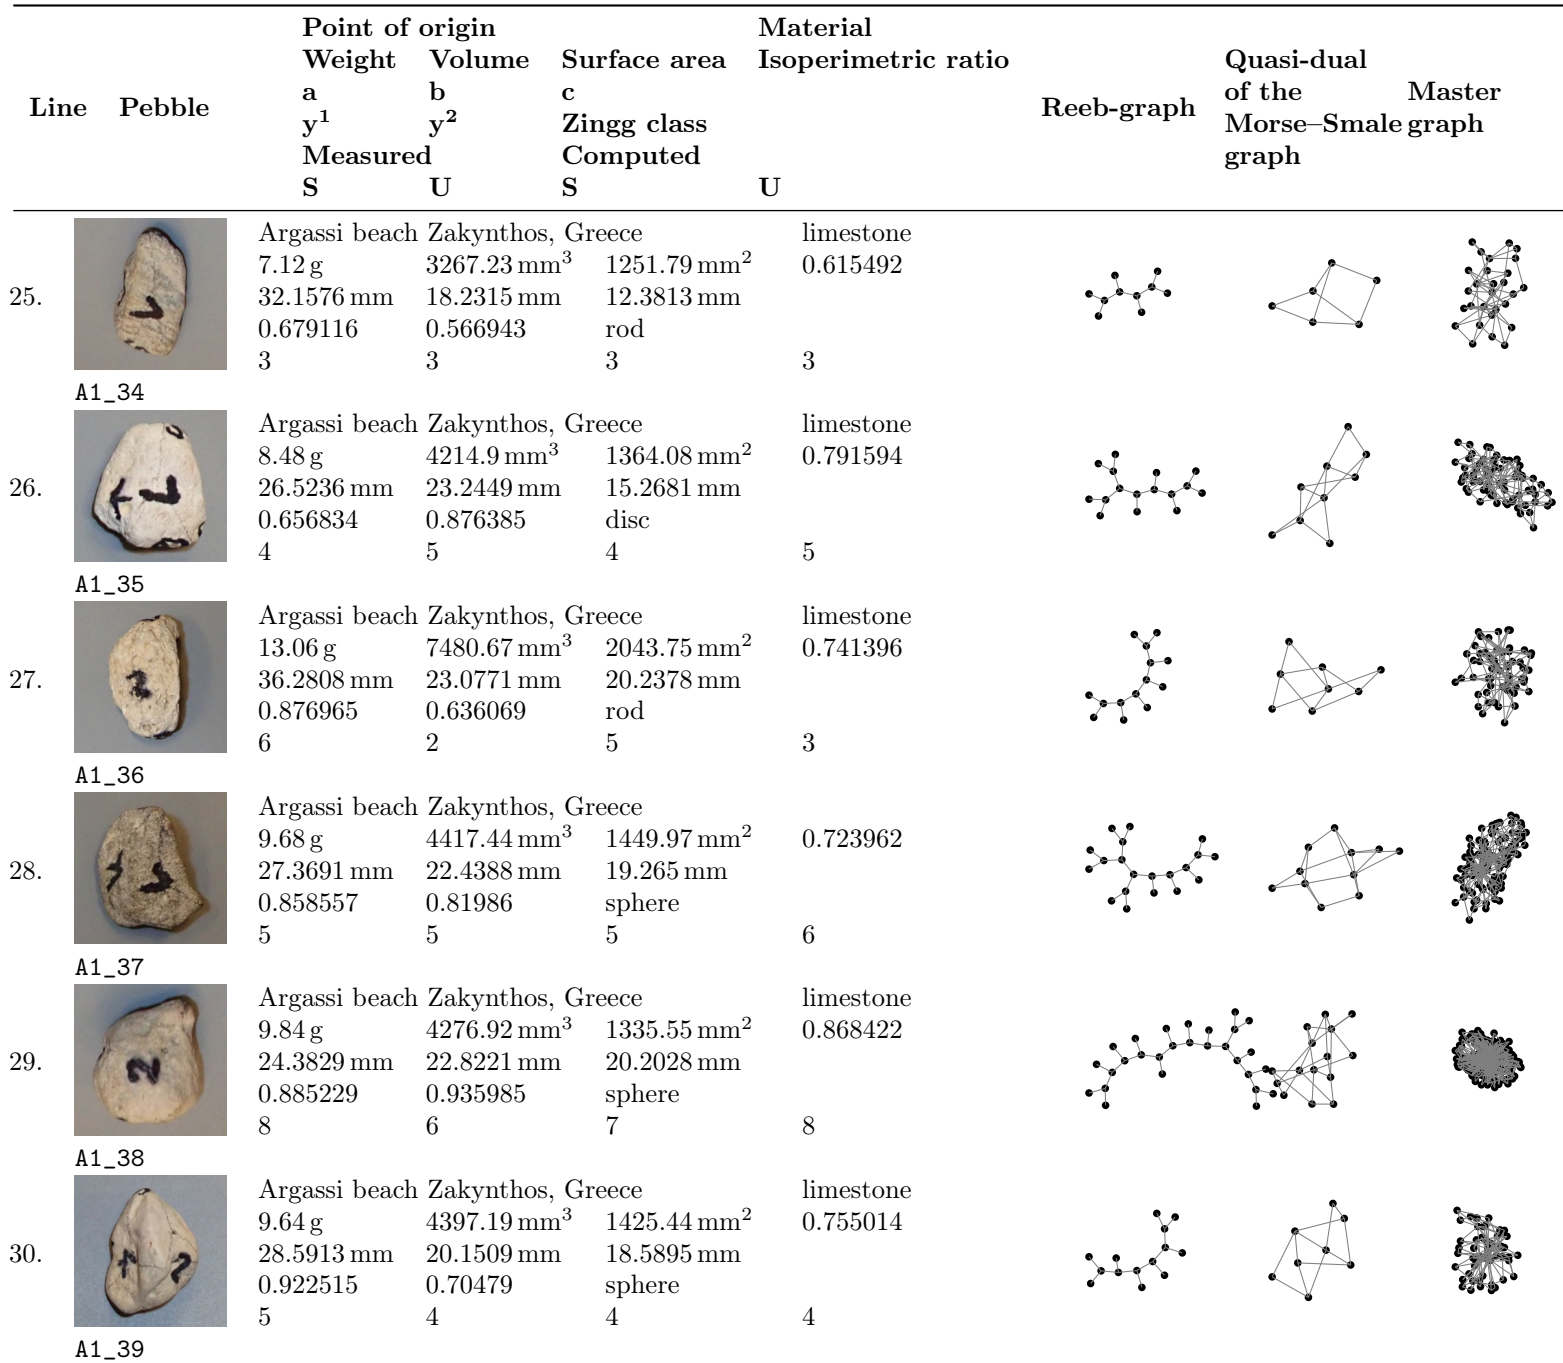   | Argassi beach<br>8.48 g<br>26.5236 mm<br>0.656834<br>4  | Zakynthos, Greece<br>4214.9 mm <sup>3</sup><br>23.2449 mm<br>0.876385<br>5  | limestone<br>1364.08 mm <sup>2</sup><br>15.2681 mm<br>disc<br>4   | 0.791594 | 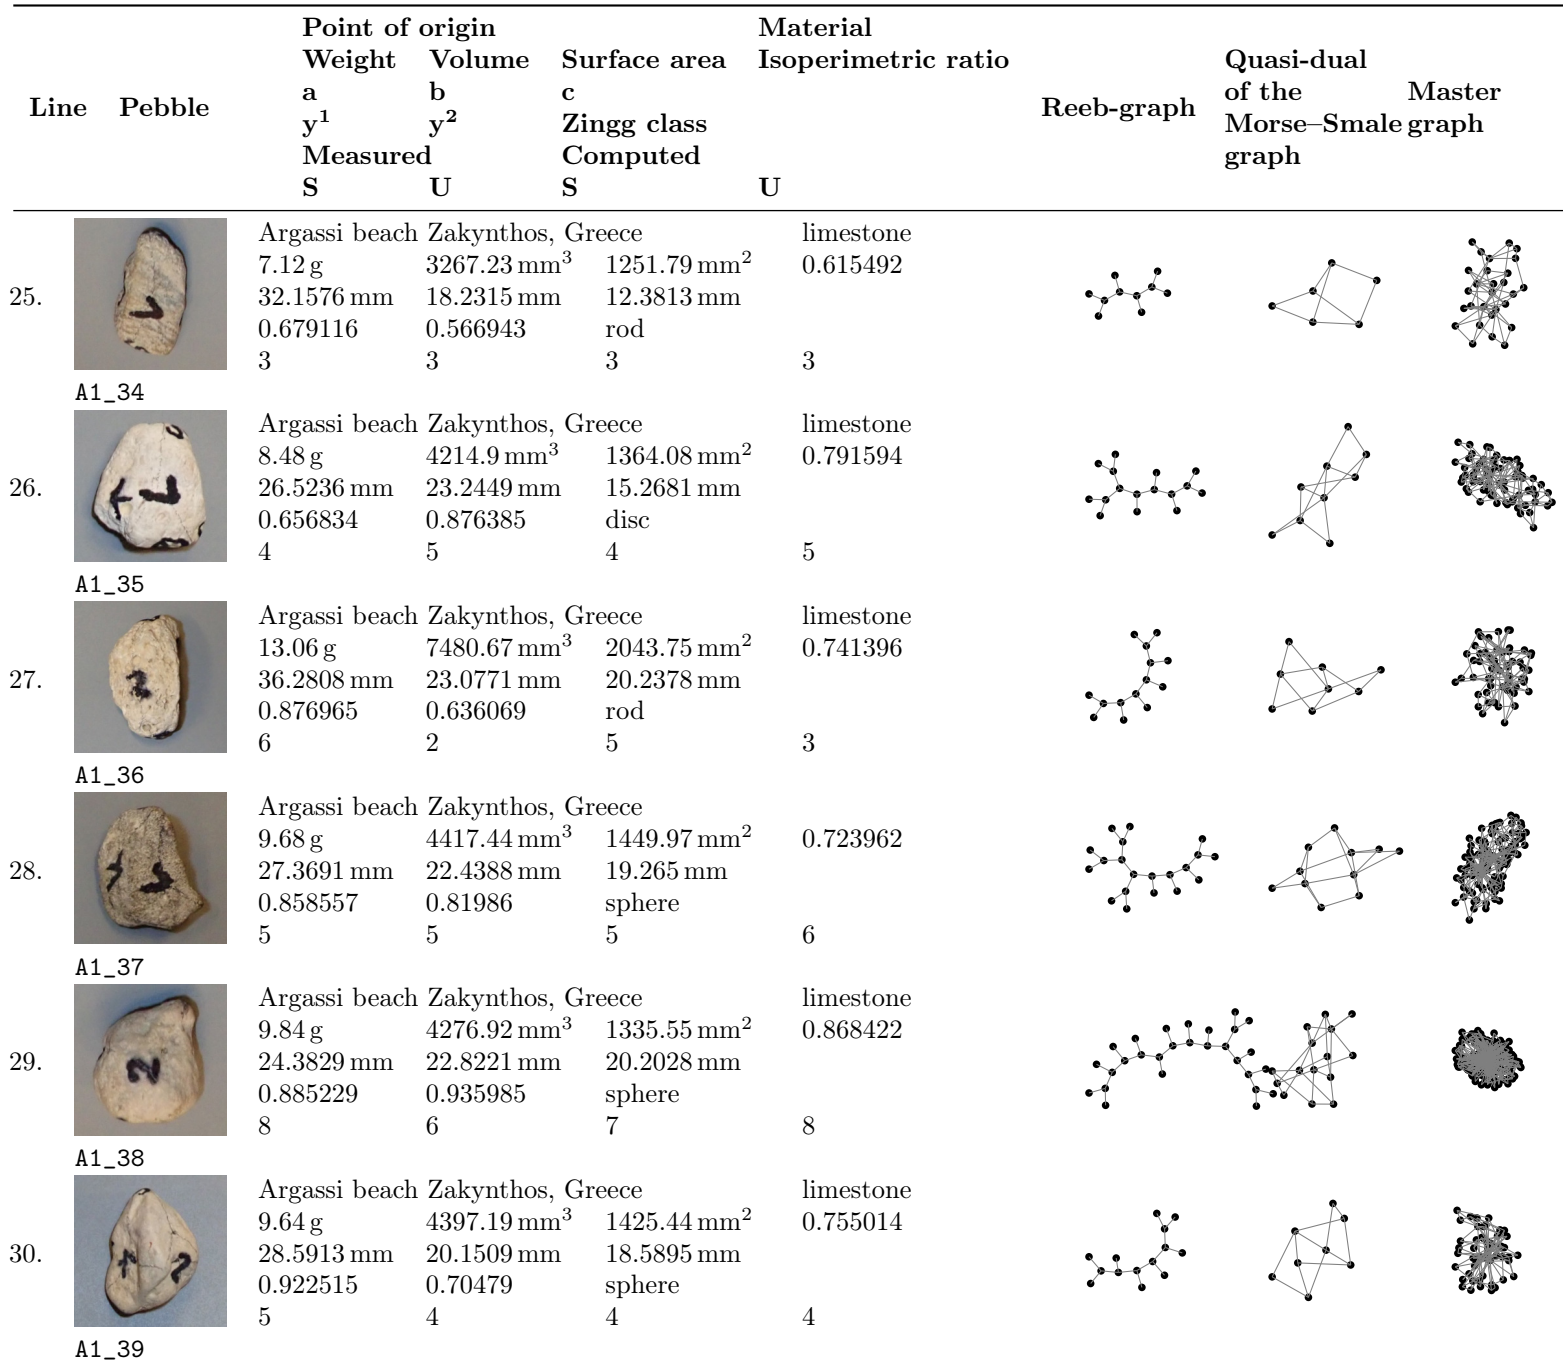   | 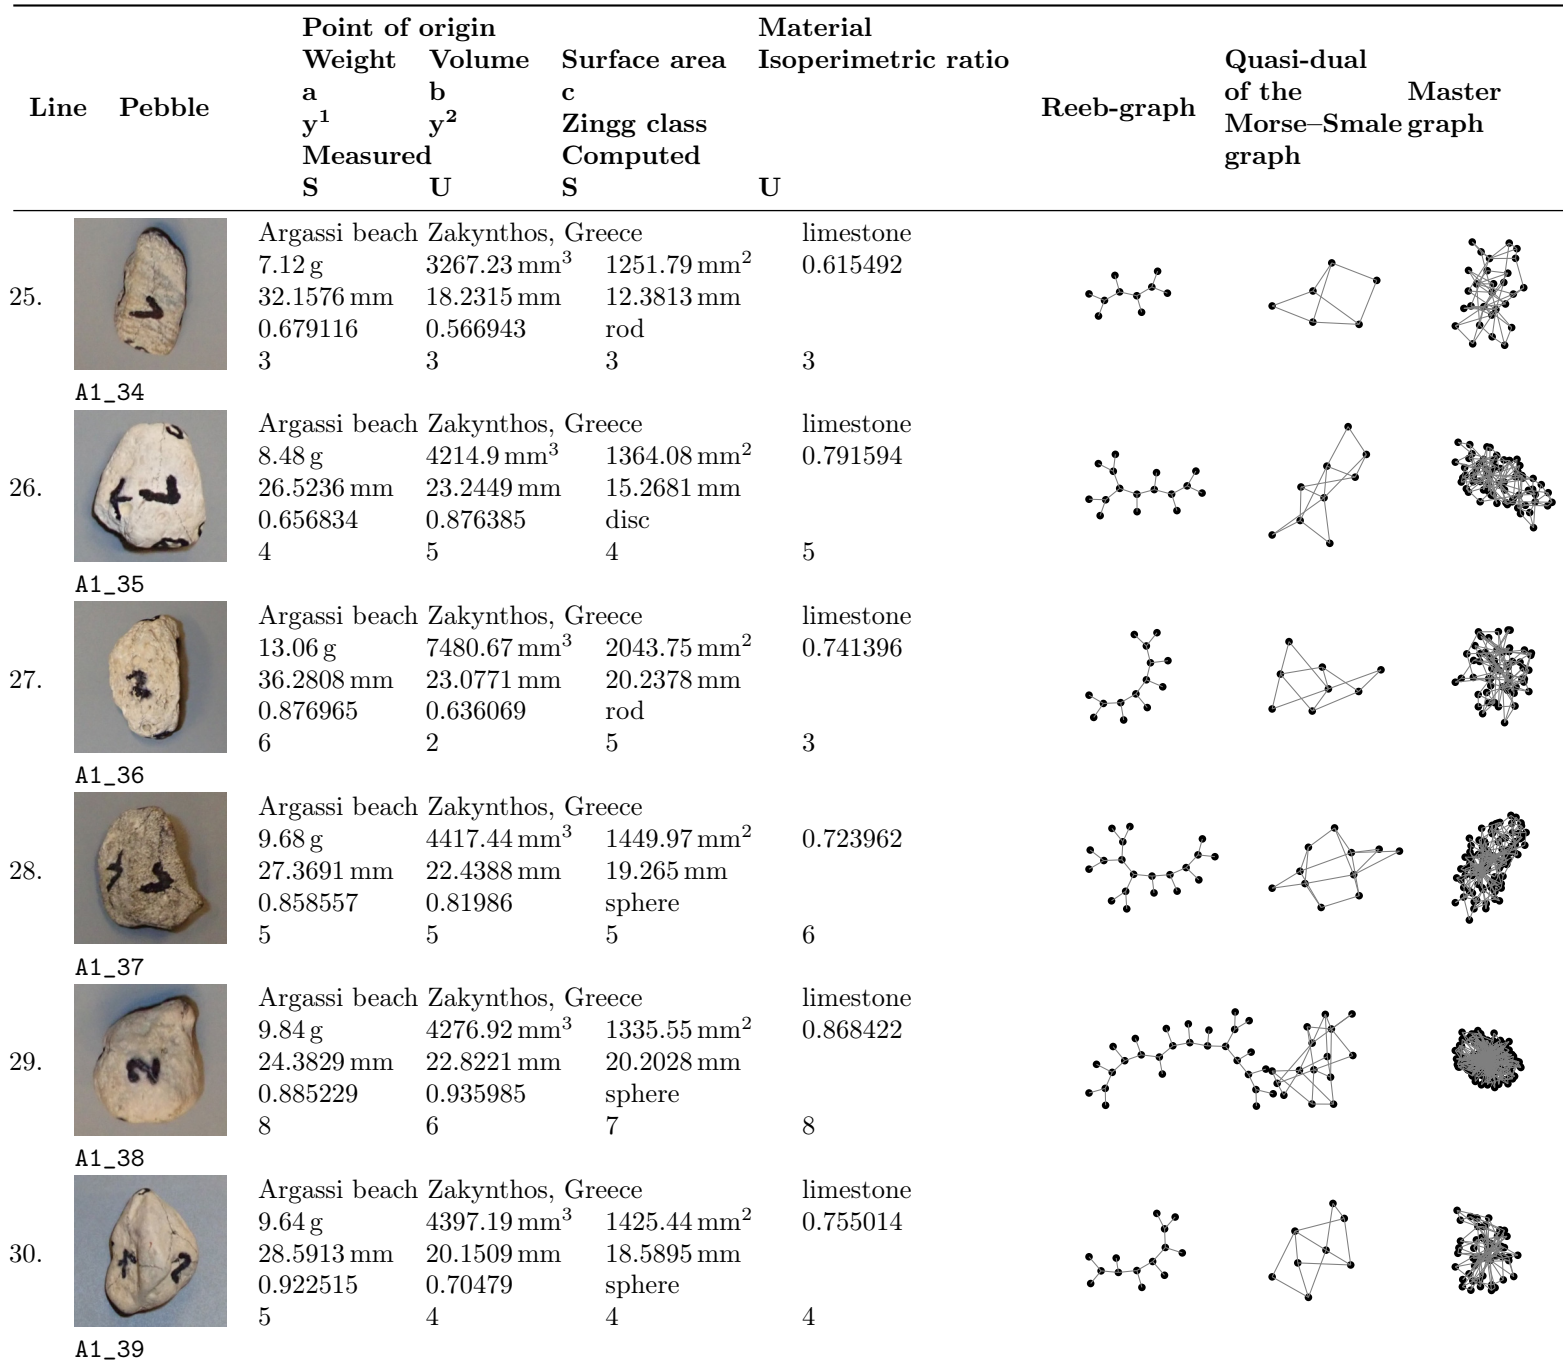   | 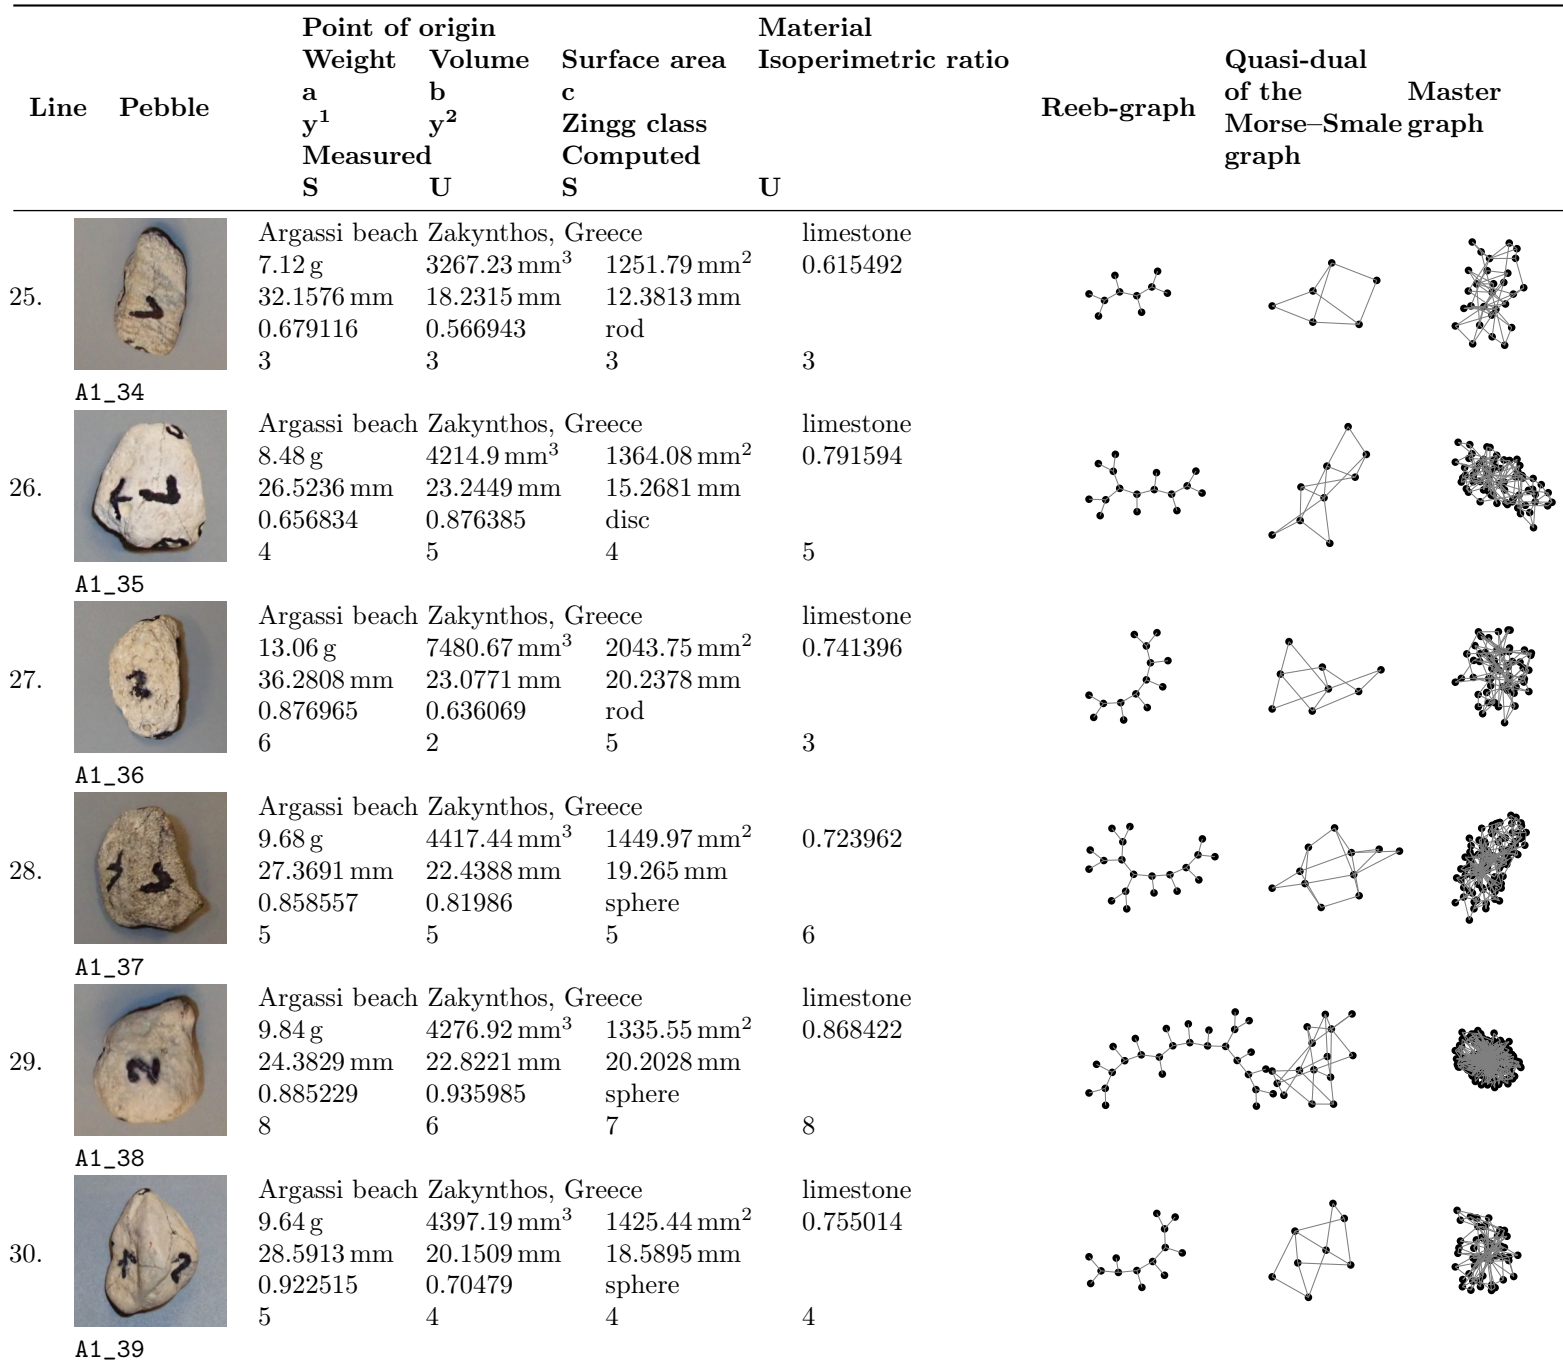   |
|      | A1_35                                                                               |                                                         |                                                                             |                                                                   |          |                                                                                       |                                                                                       |                                                                                       |
| 27.  | 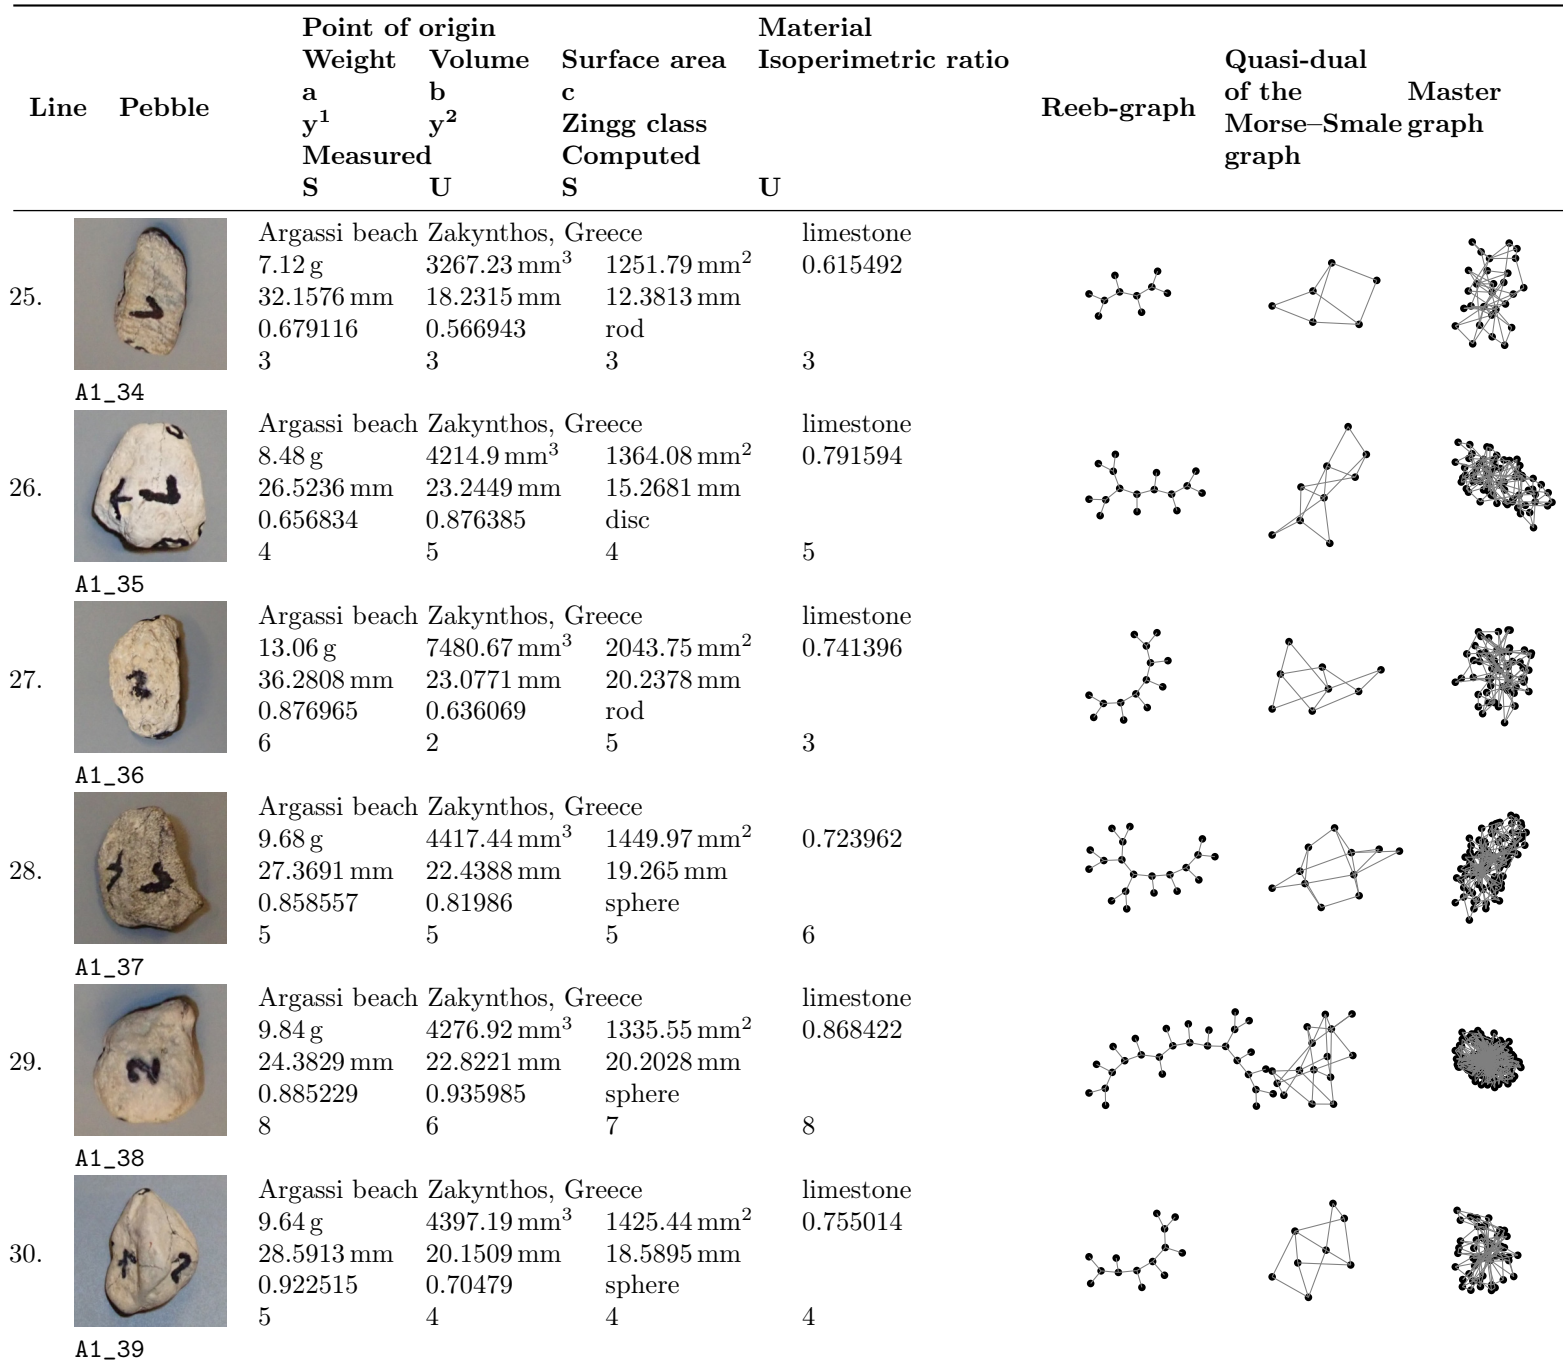   | Argassi beach<br>13.06 g<br>36.2808 mm<br>0.876965<br>6 | Zakynthos, Greece<br>7480.67 mm <sup>3</sup><br>23.0771 mm<br>0.636069<br>2 | limestone<br>2043.75 mm <sup>2</sup><br>20.2378 mm<br>rod<br>5    | 0.741396 | 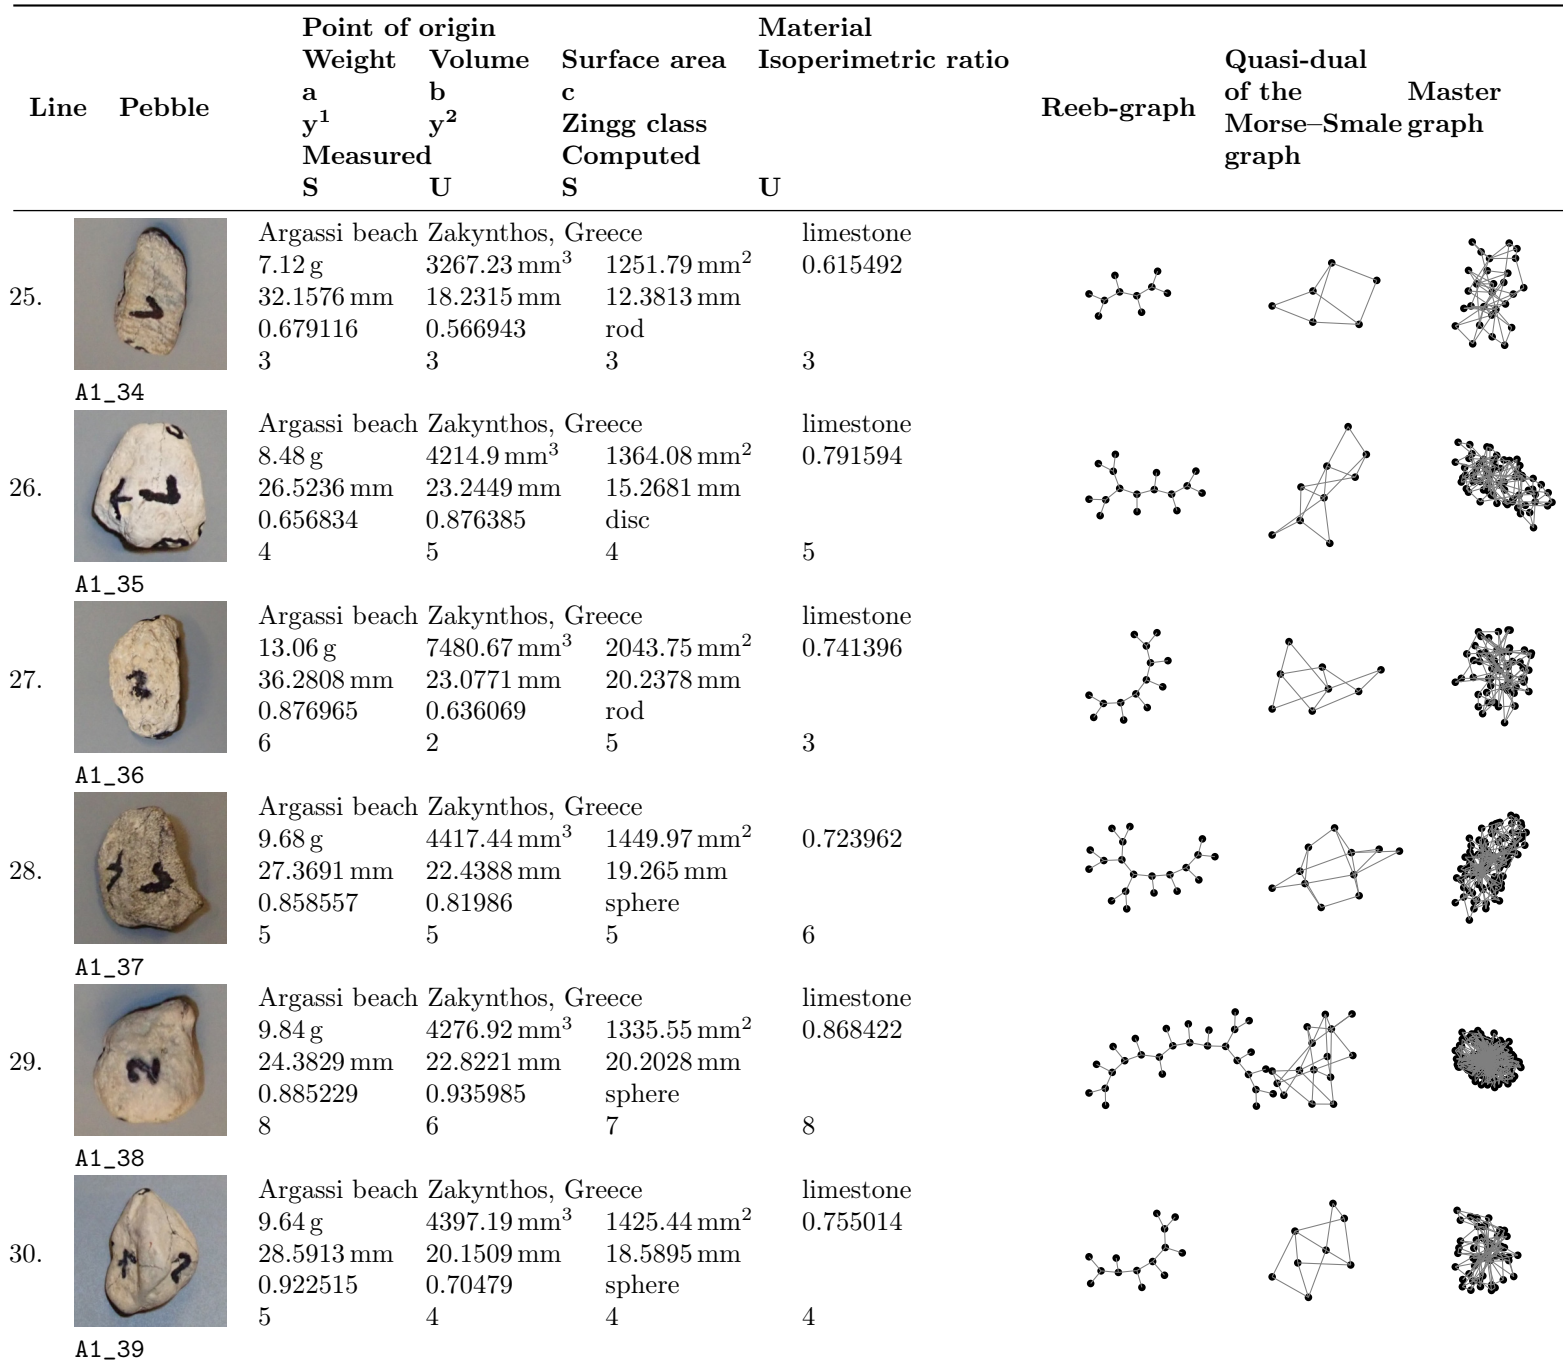   | 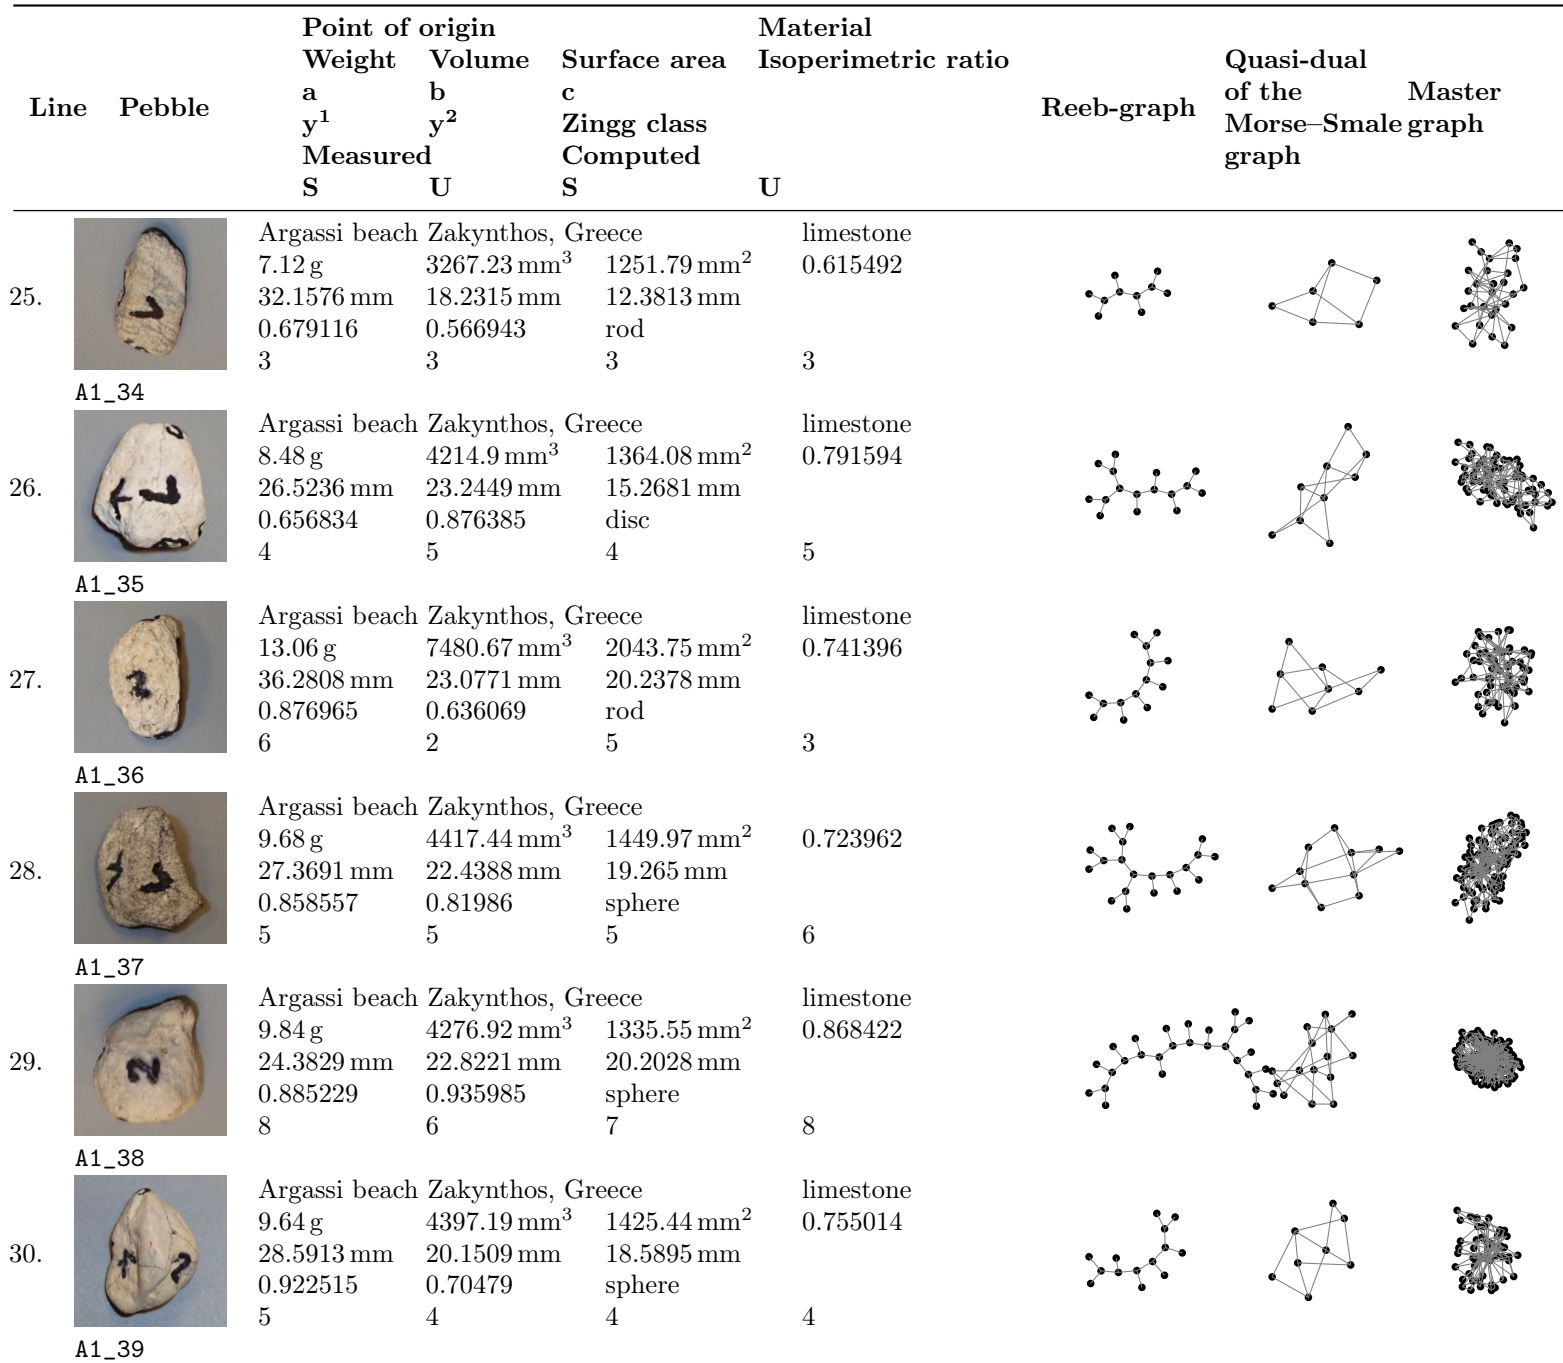   | 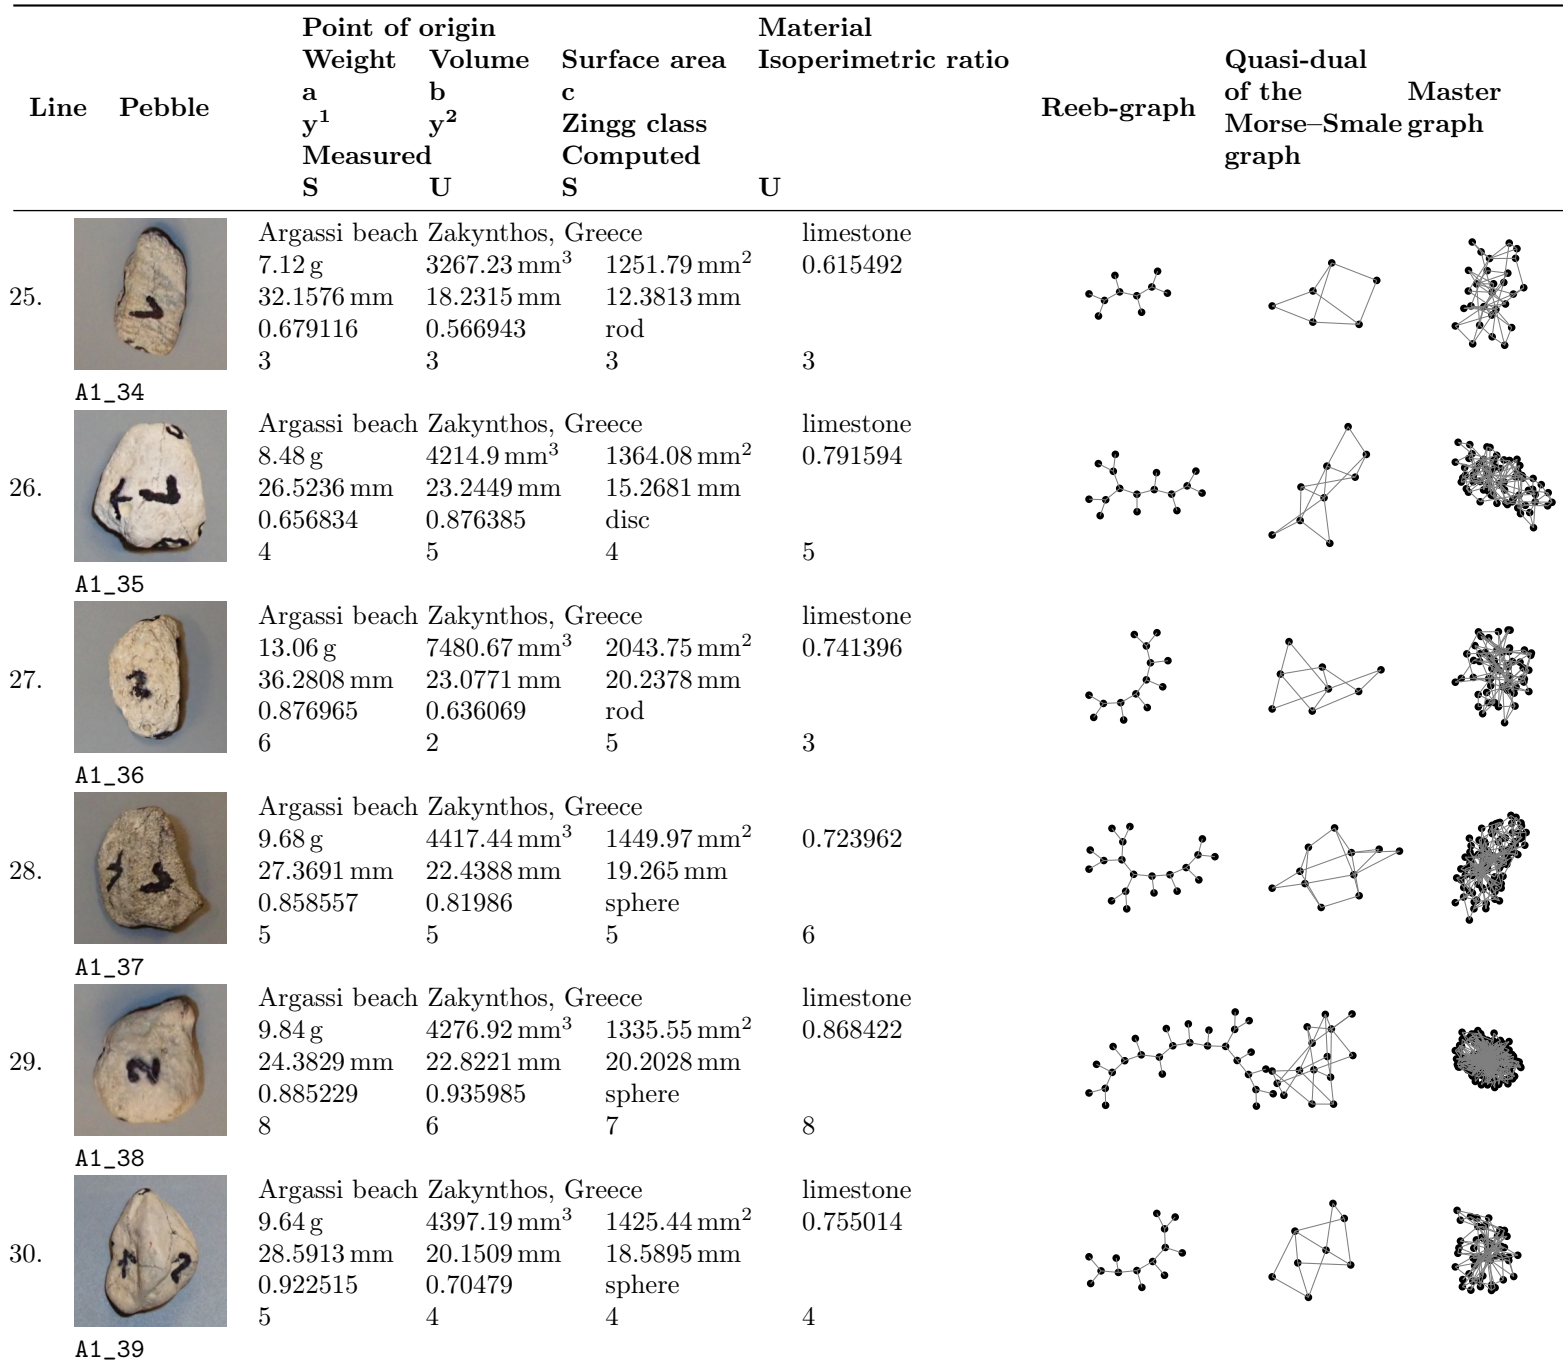   |
|      | A1_36                                                                               |                                                         |                                                                             |                                                                   |          |                                                                                       |                                                                                       |                                                                                       |
| 28.  | 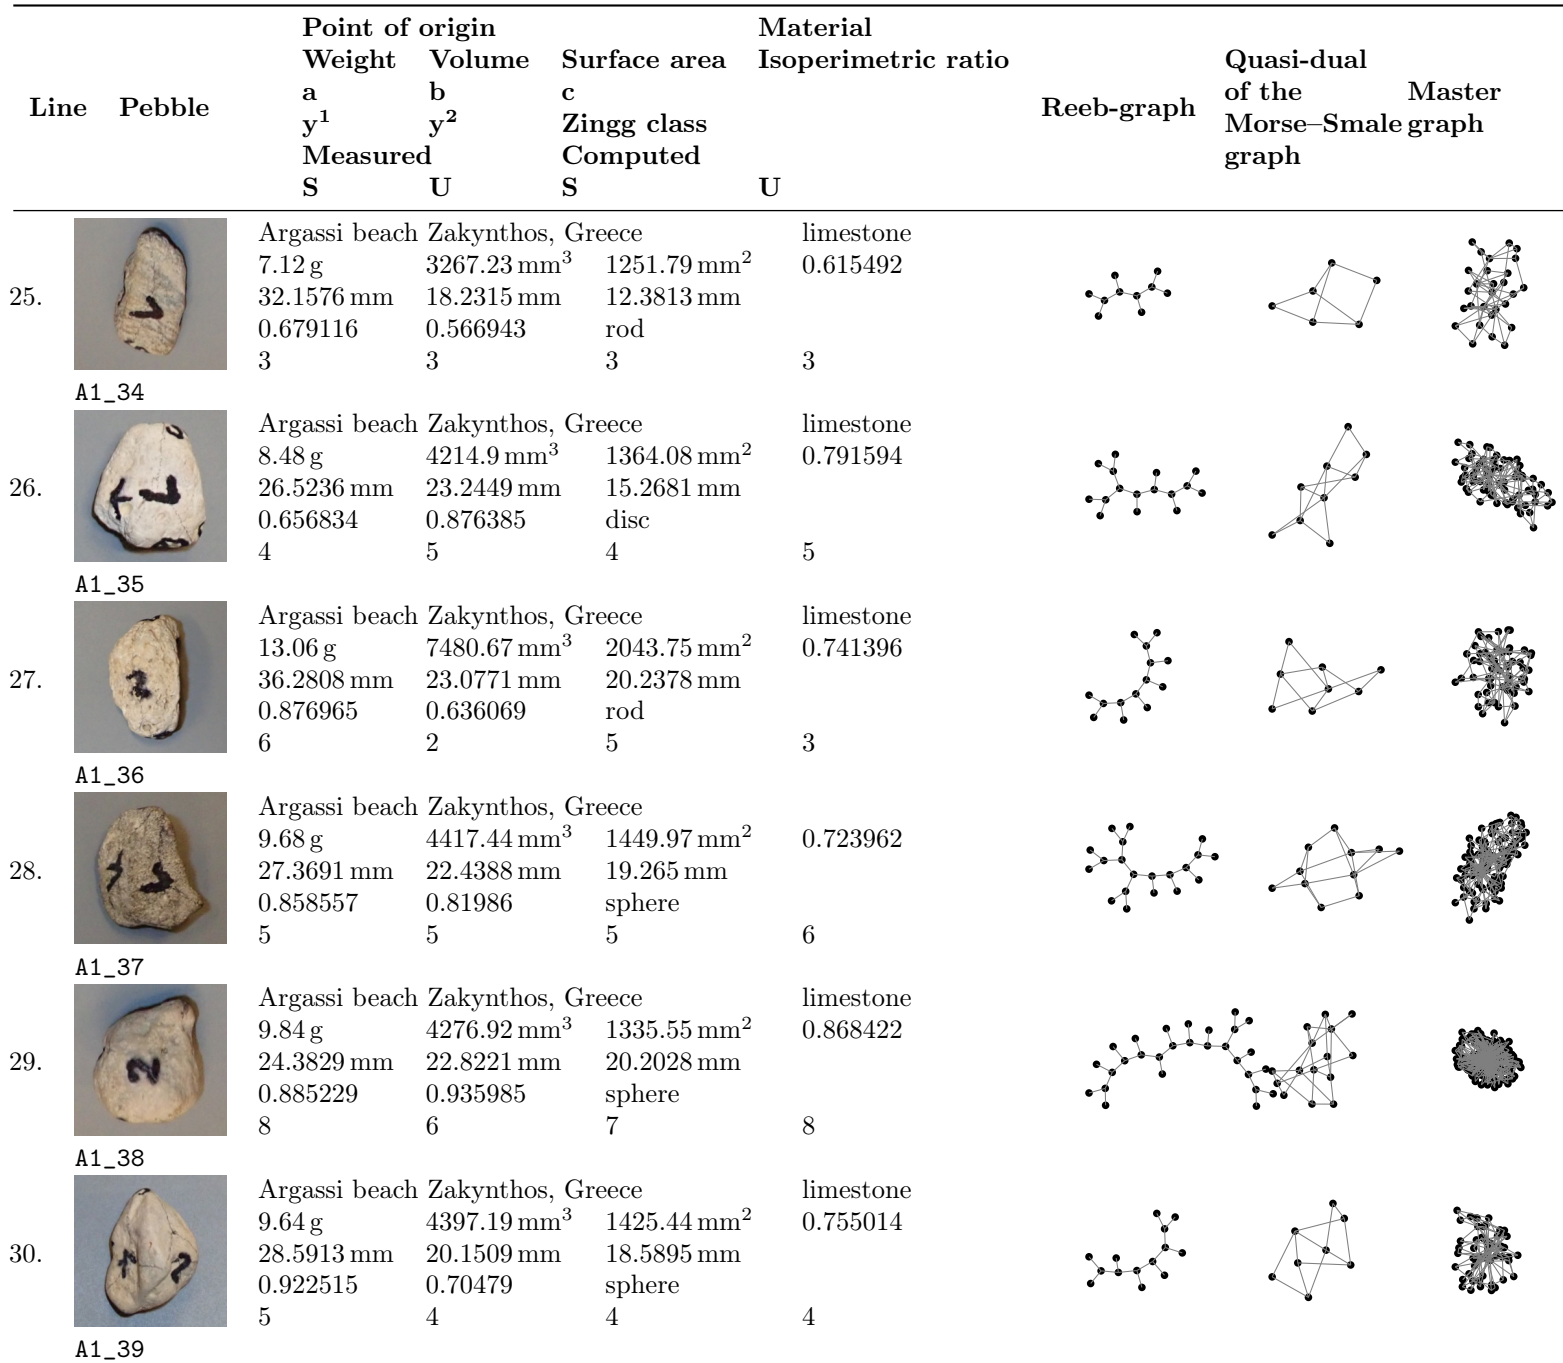  | Argassi beach<br>9.68 g<br>27.3691 mm<br>0.858557<br>5  | Zakynthos, Greece<br>4417.44 mm <sup>3</sup><br>22.4388 mm<br>0.81986<br>5  | limestone<br>1449.97 mm <sup>2</sup><br>19.265 mm<br>sphere<br>5  | 0.723962 | 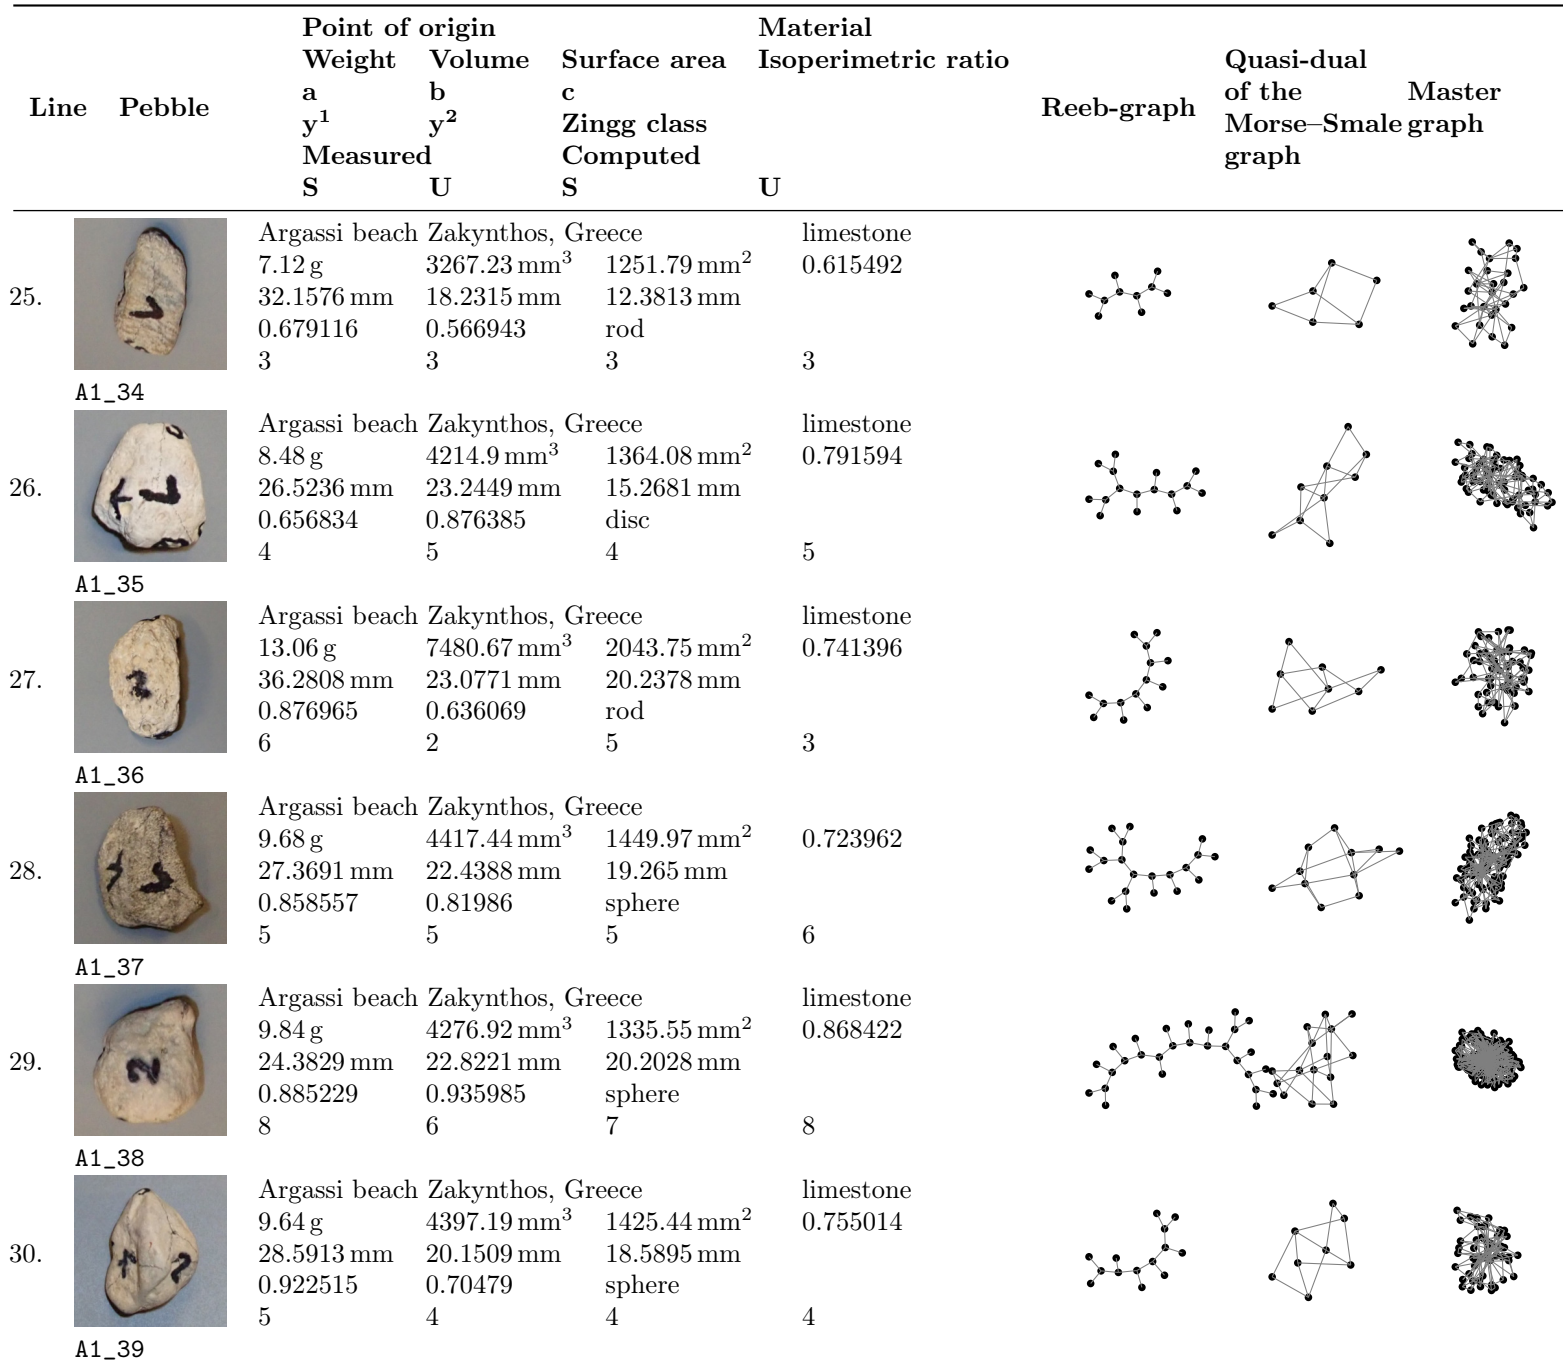  | 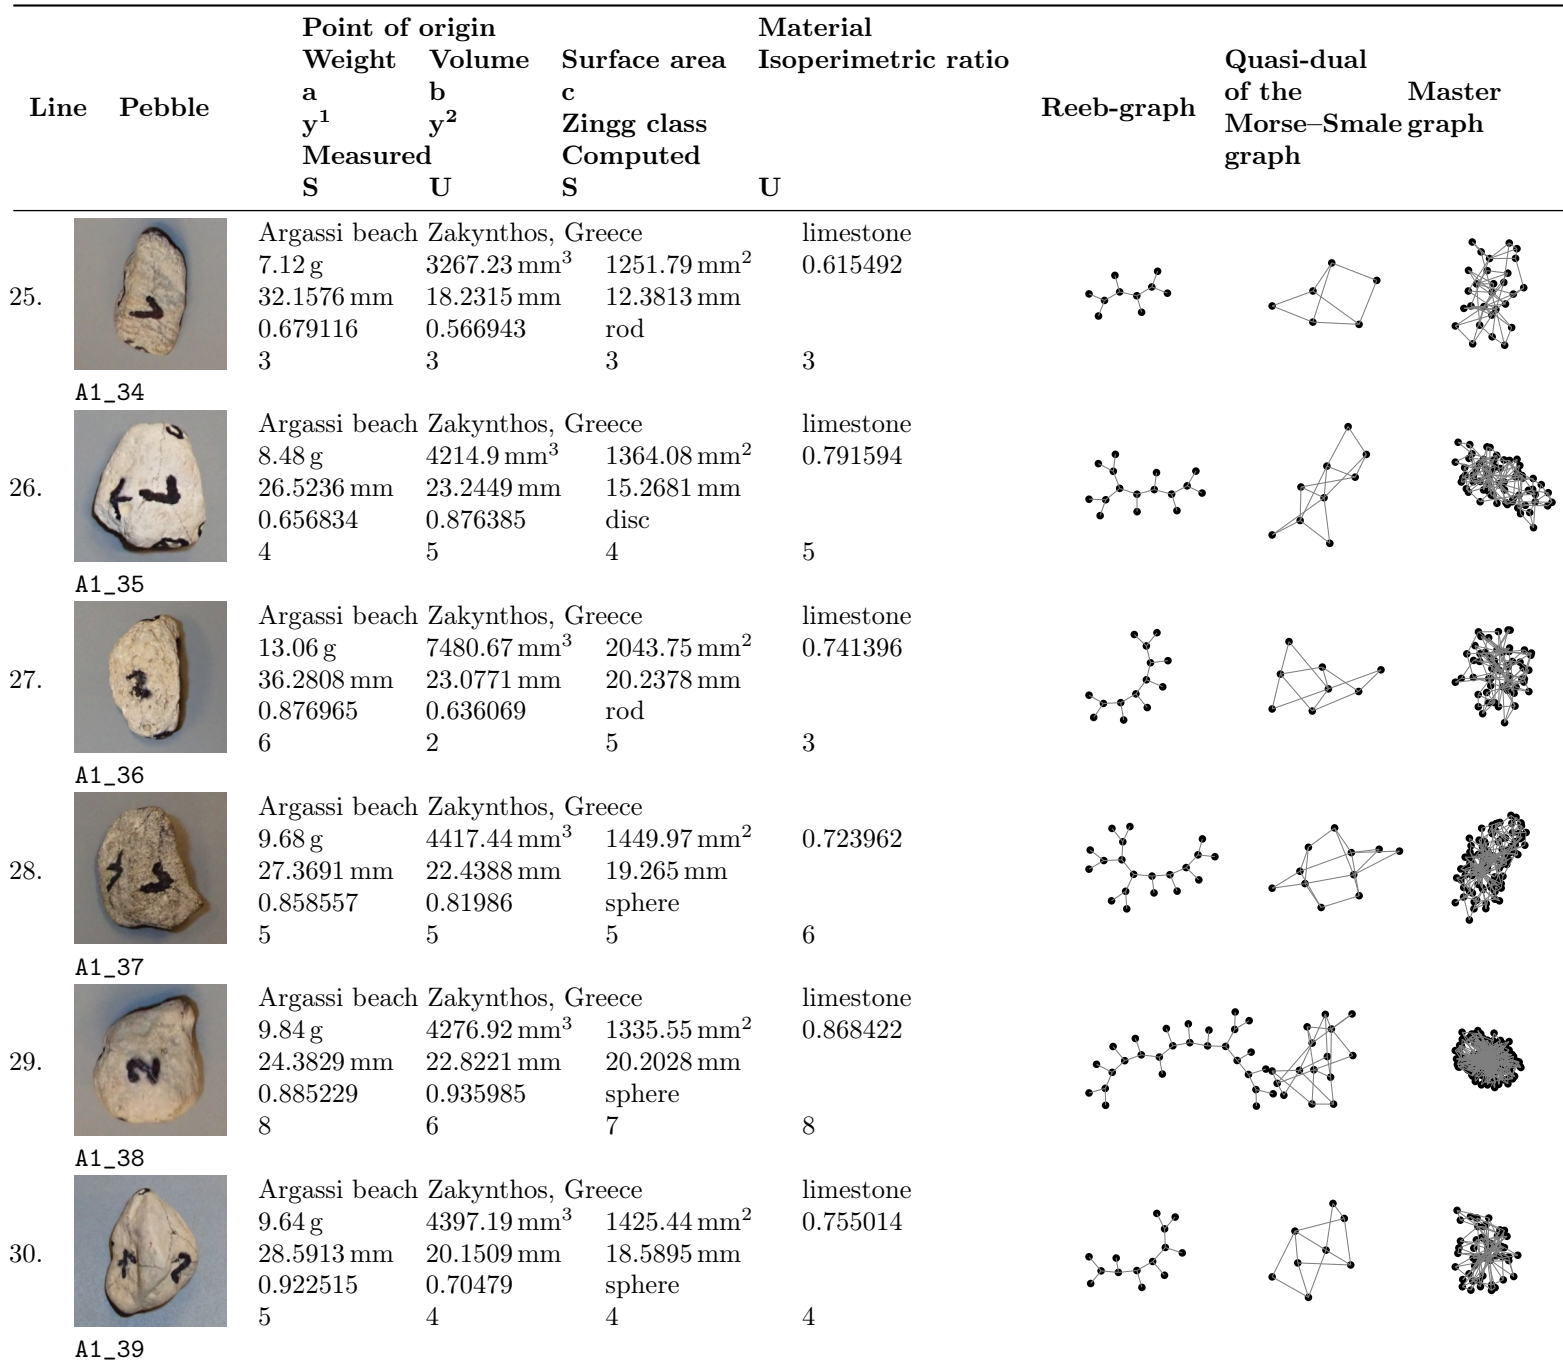  | 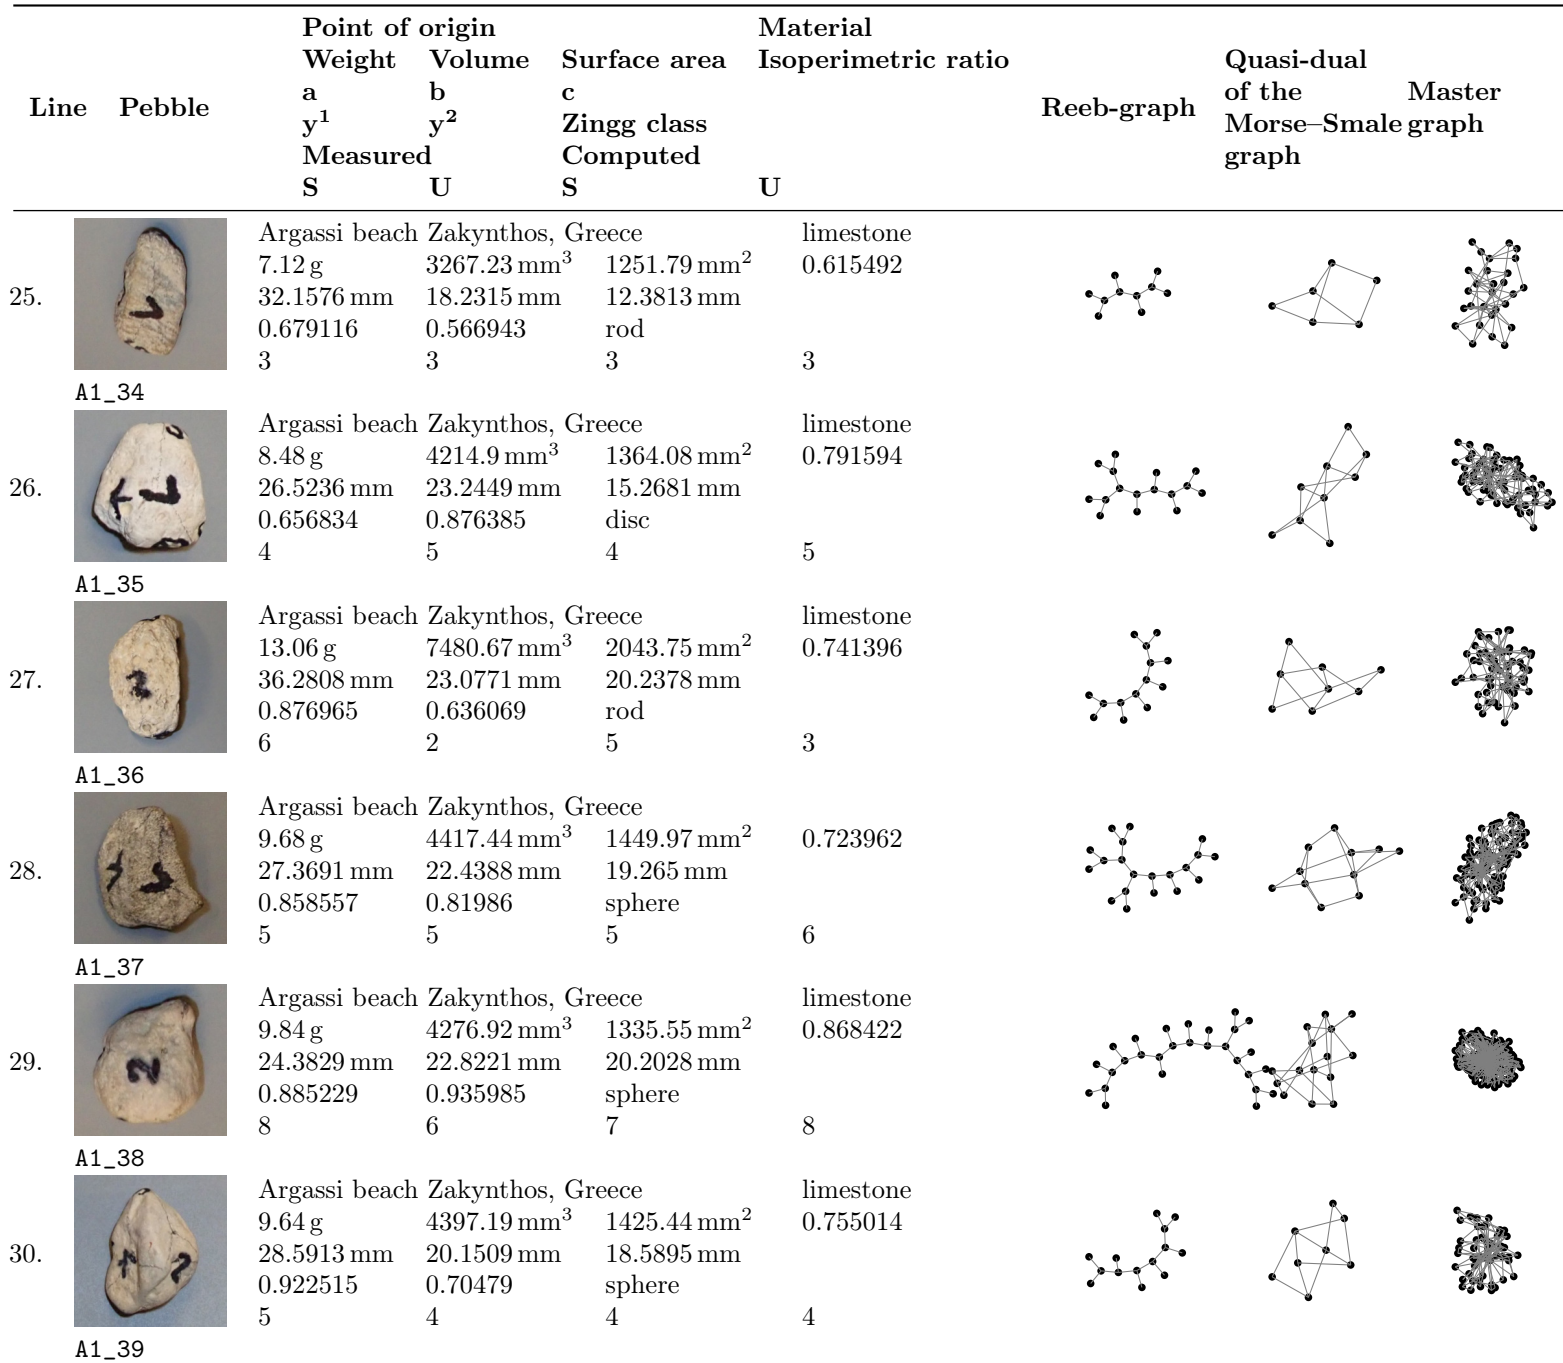  |
|      | A1_37                                                                               |                                                         |                                                                             |                                                                   |          |                                                                                       |                                                                                       |                                                                                       |
| 29.  | 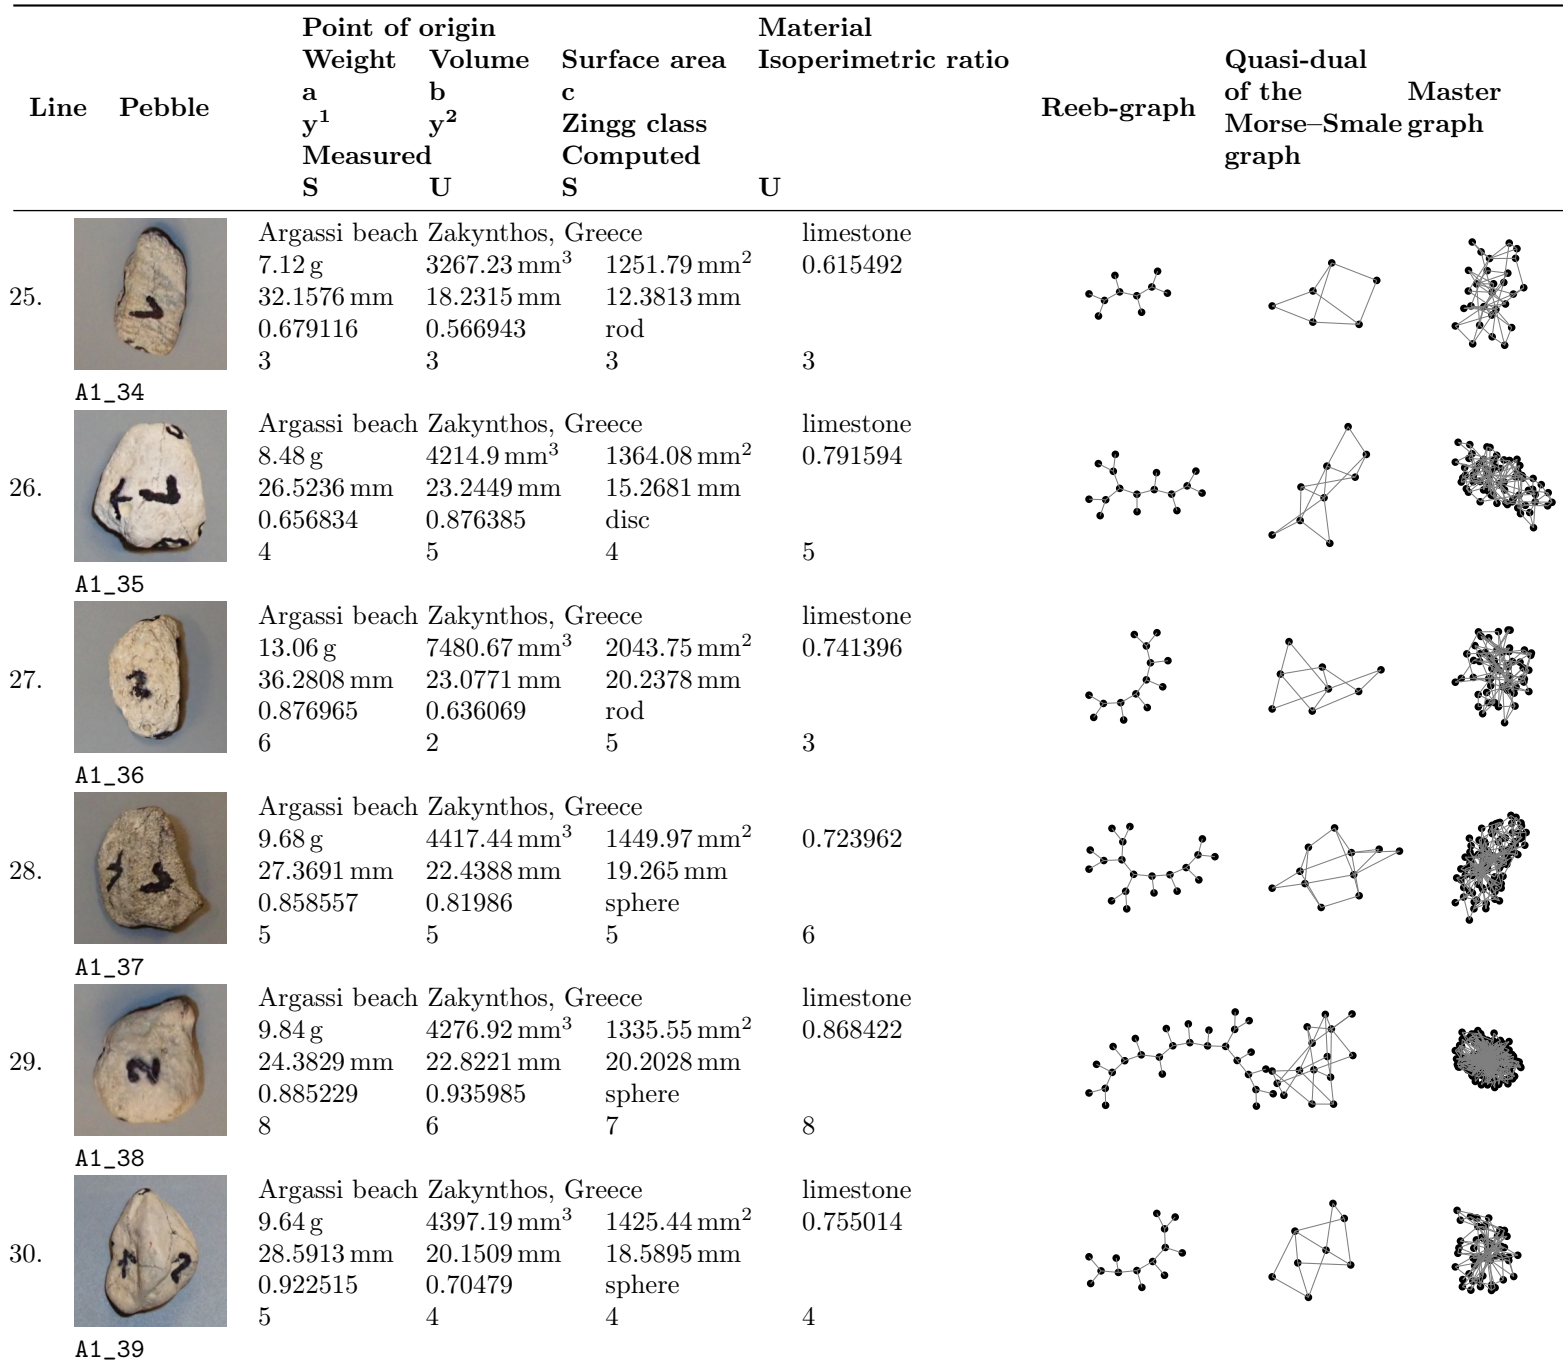 | Argassi beach<br>9.84 g<br>24.3829 mm<br>0.885229<br>8  | Zakynthos, Greece<br>4276.92 mm <sup>3</sup><br>22.8221 mm<br>0.935985<br>6 | limestone<br>1335.55 mm <sup>2</sup><br>20.2028 mm<br>sphere<br>7 | 0.868422 | 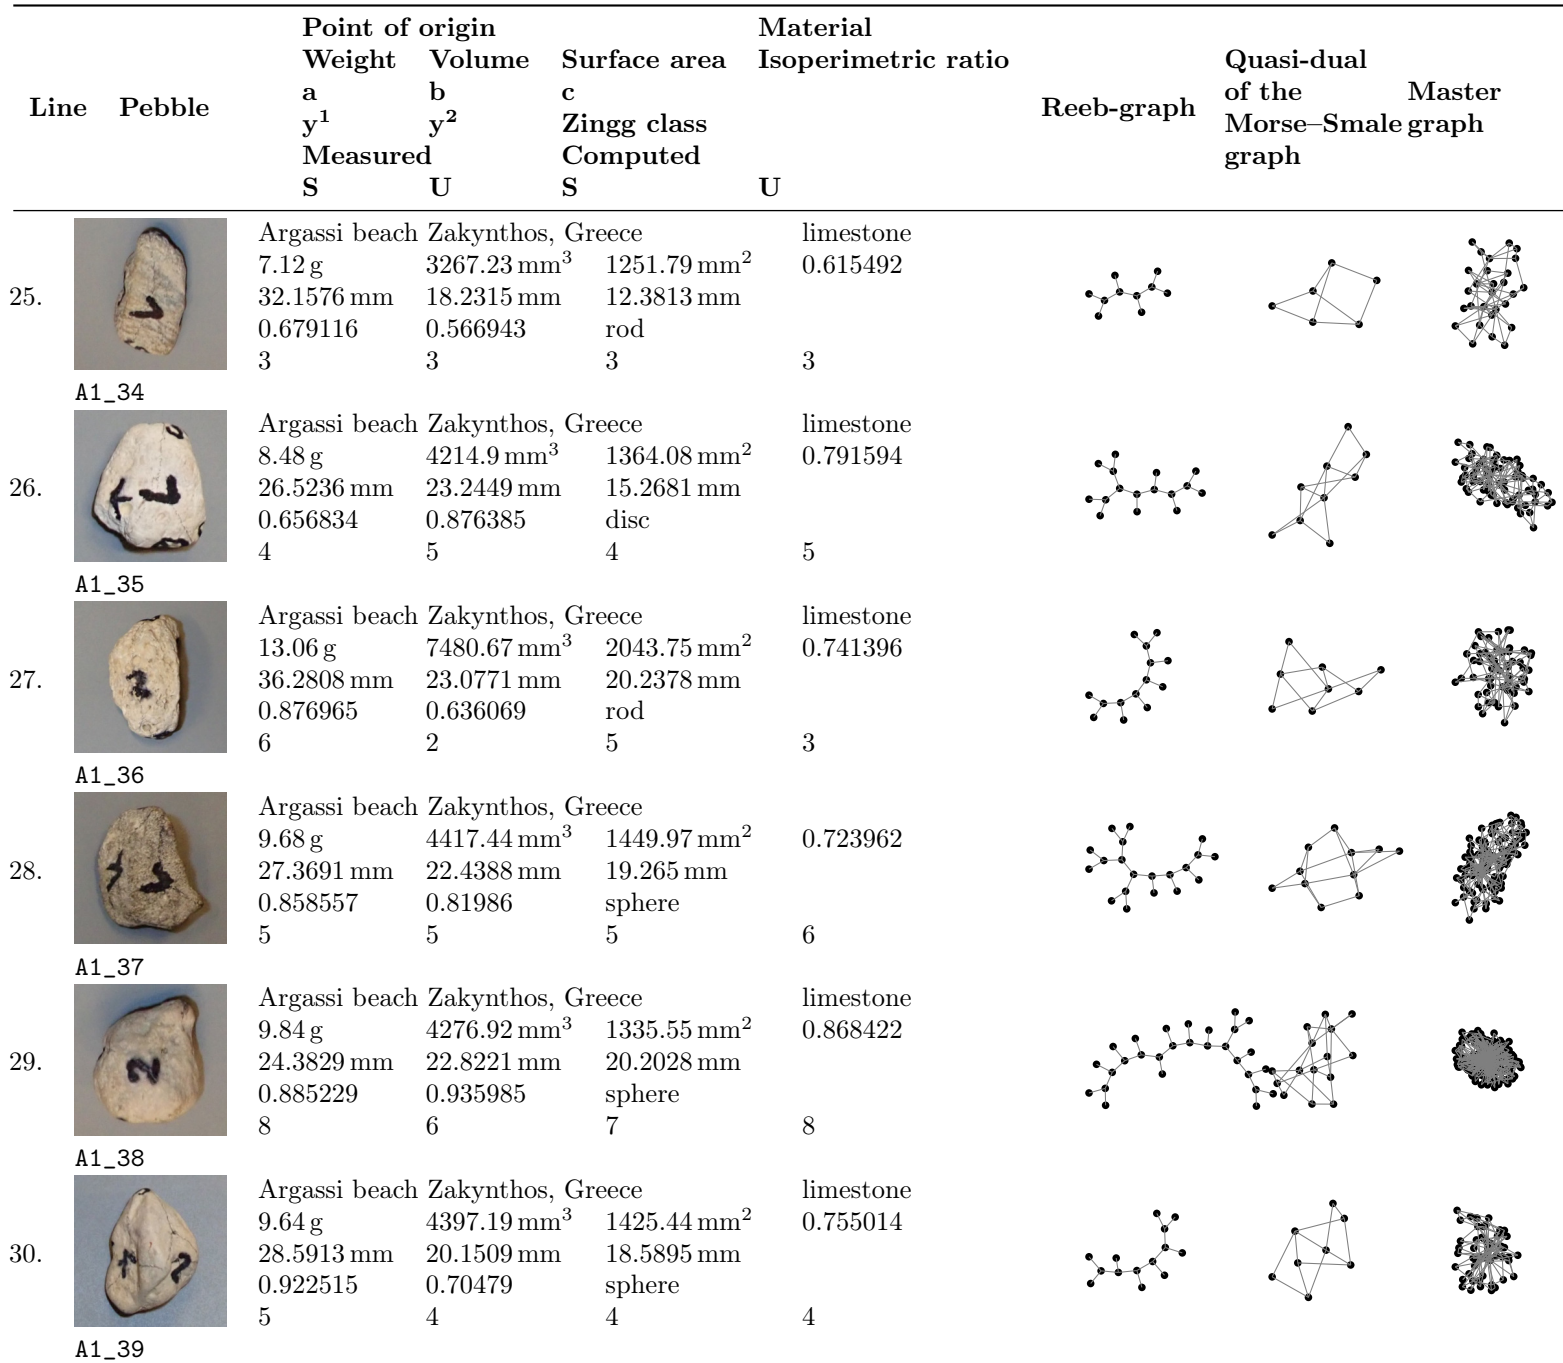 | 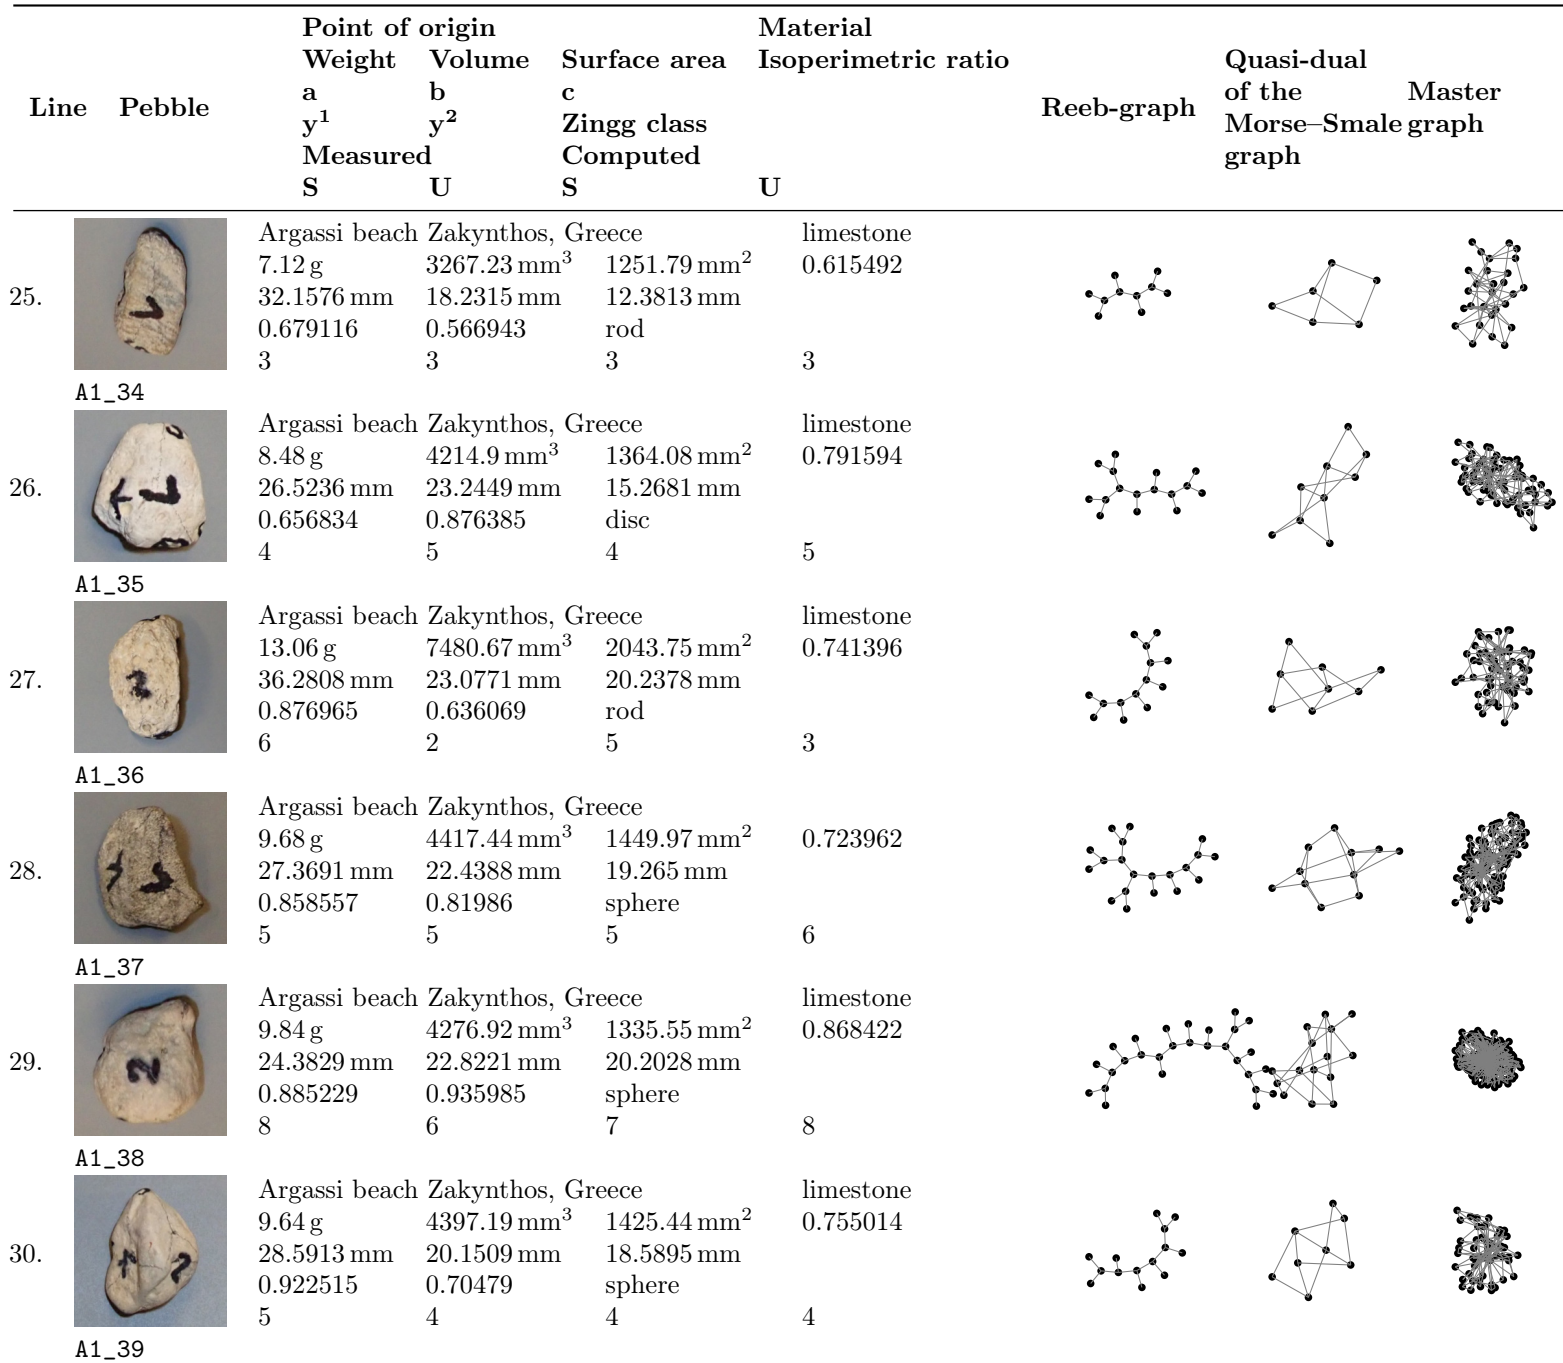 | 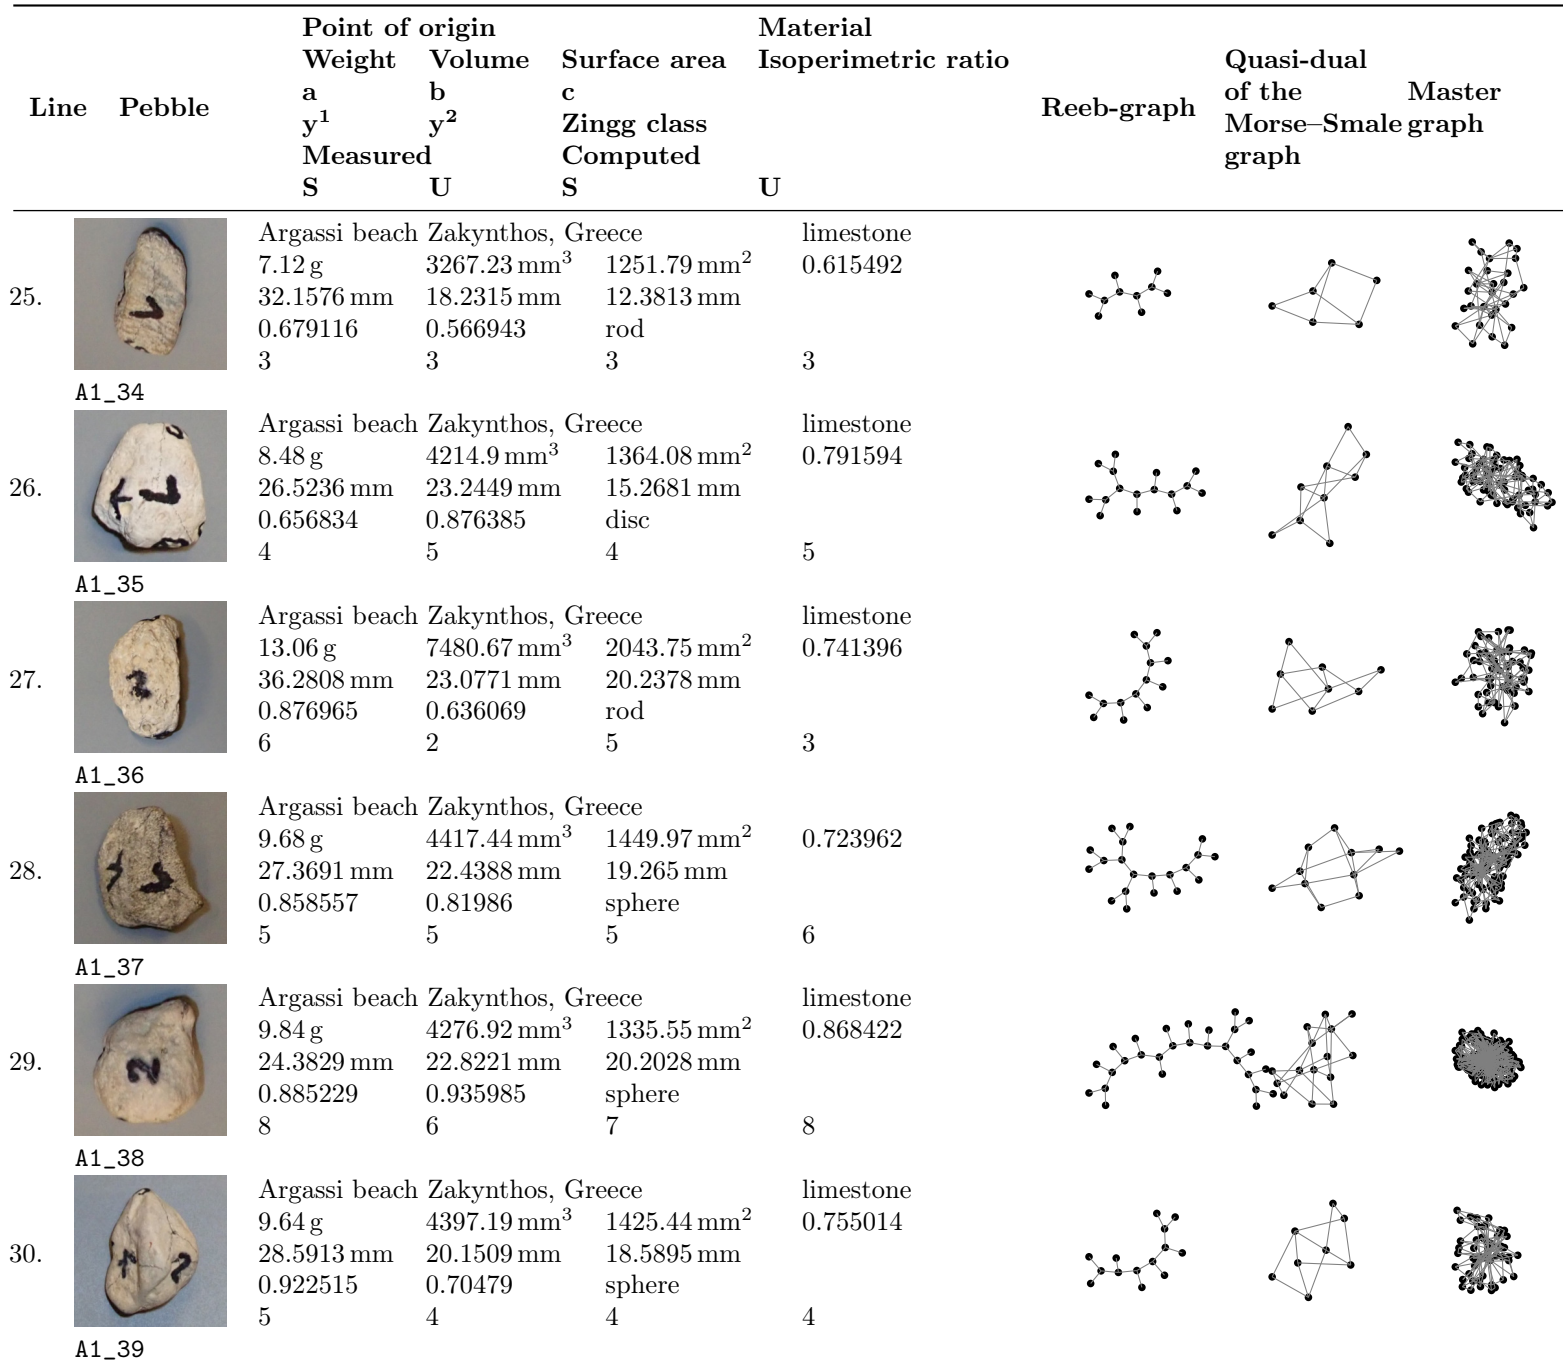 |
|      | A1_38                                                                               |                                                         |                                                                             |                                                                   |          |                                                                                       |                                                                                       |                                                                                       |
| 30.  | 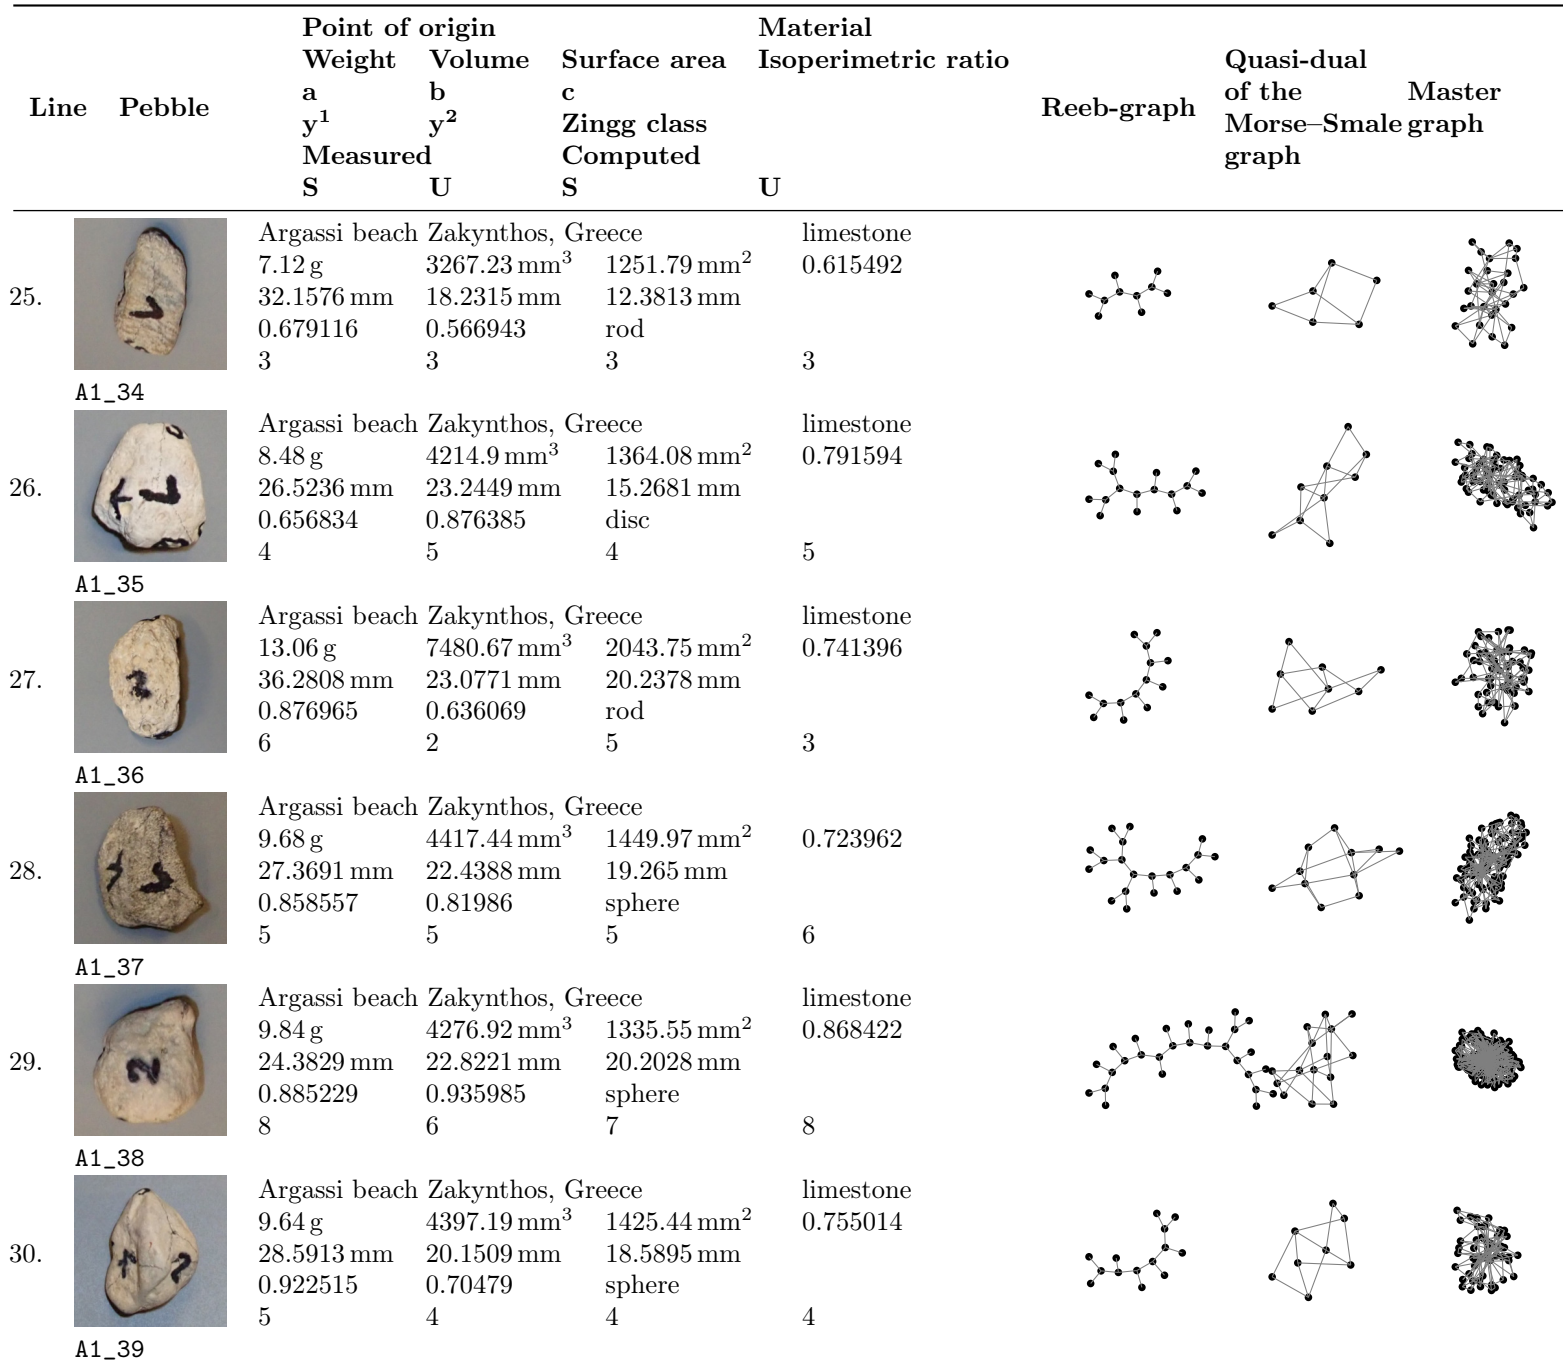 | Argassi beach<br>9.64 g<br>28.5913 mm<br>0.922515<br>5  | Zakynthos, Greece<br>4397.19 mm <sup>3</sup><br>20.1509 mm<br>0.70479<br>4  | limestone<br>1425.44 mm <sup>2</sup><br>18.5895 mm<br>sphere<br>4 | 0.755014 | 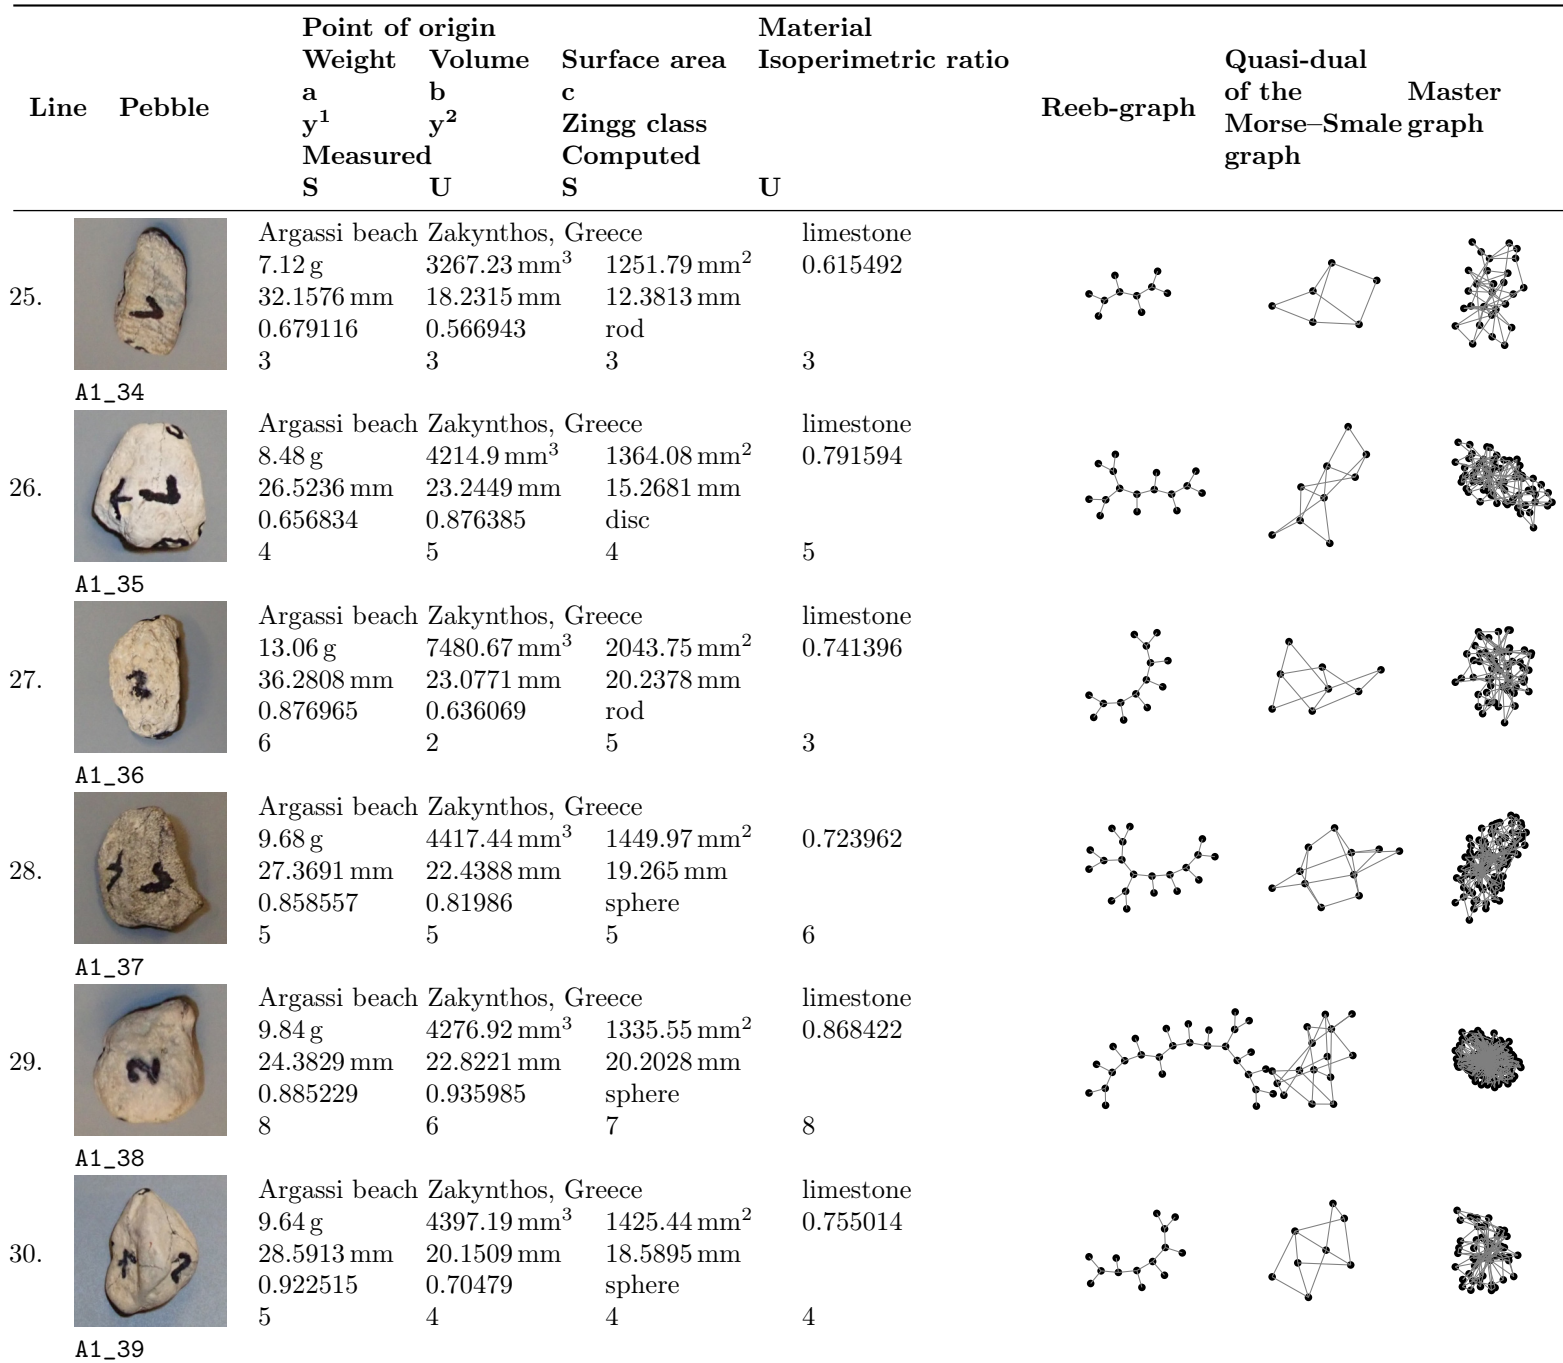 | 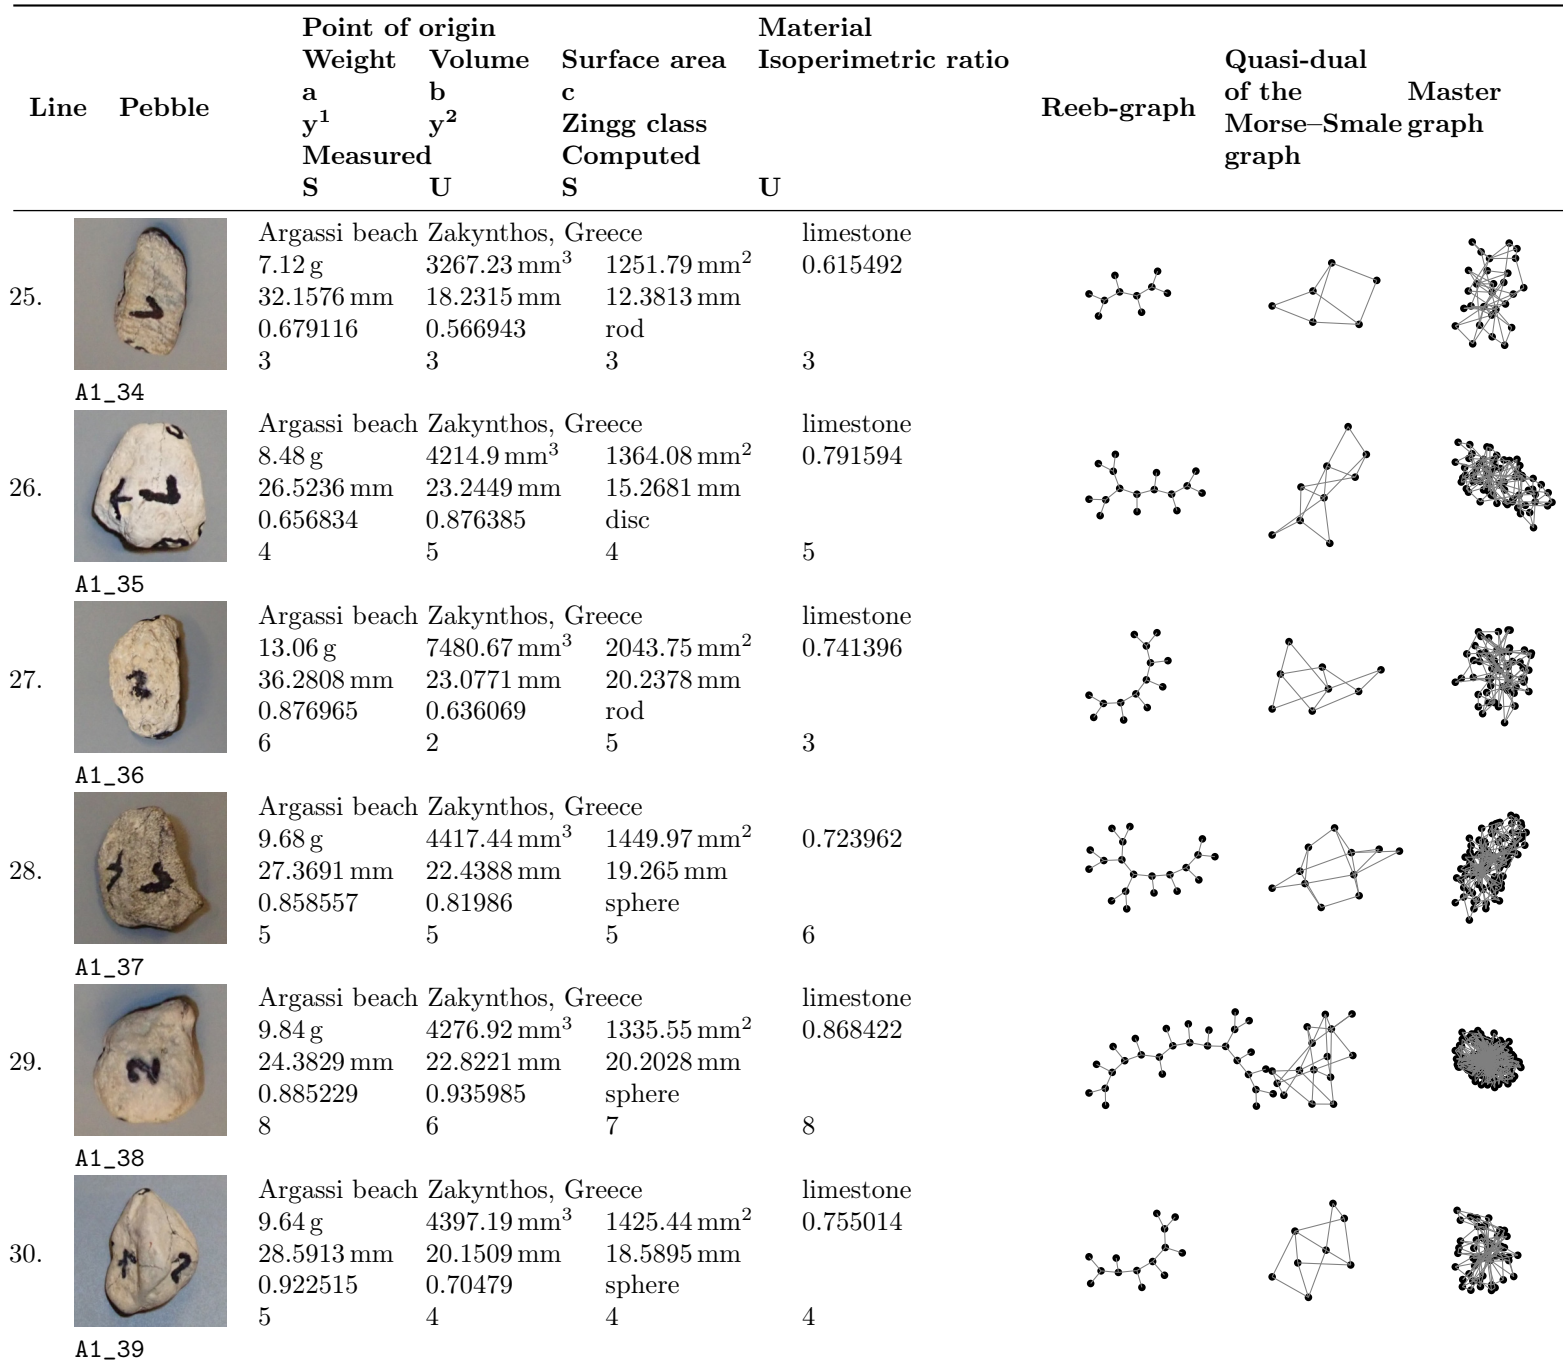 | 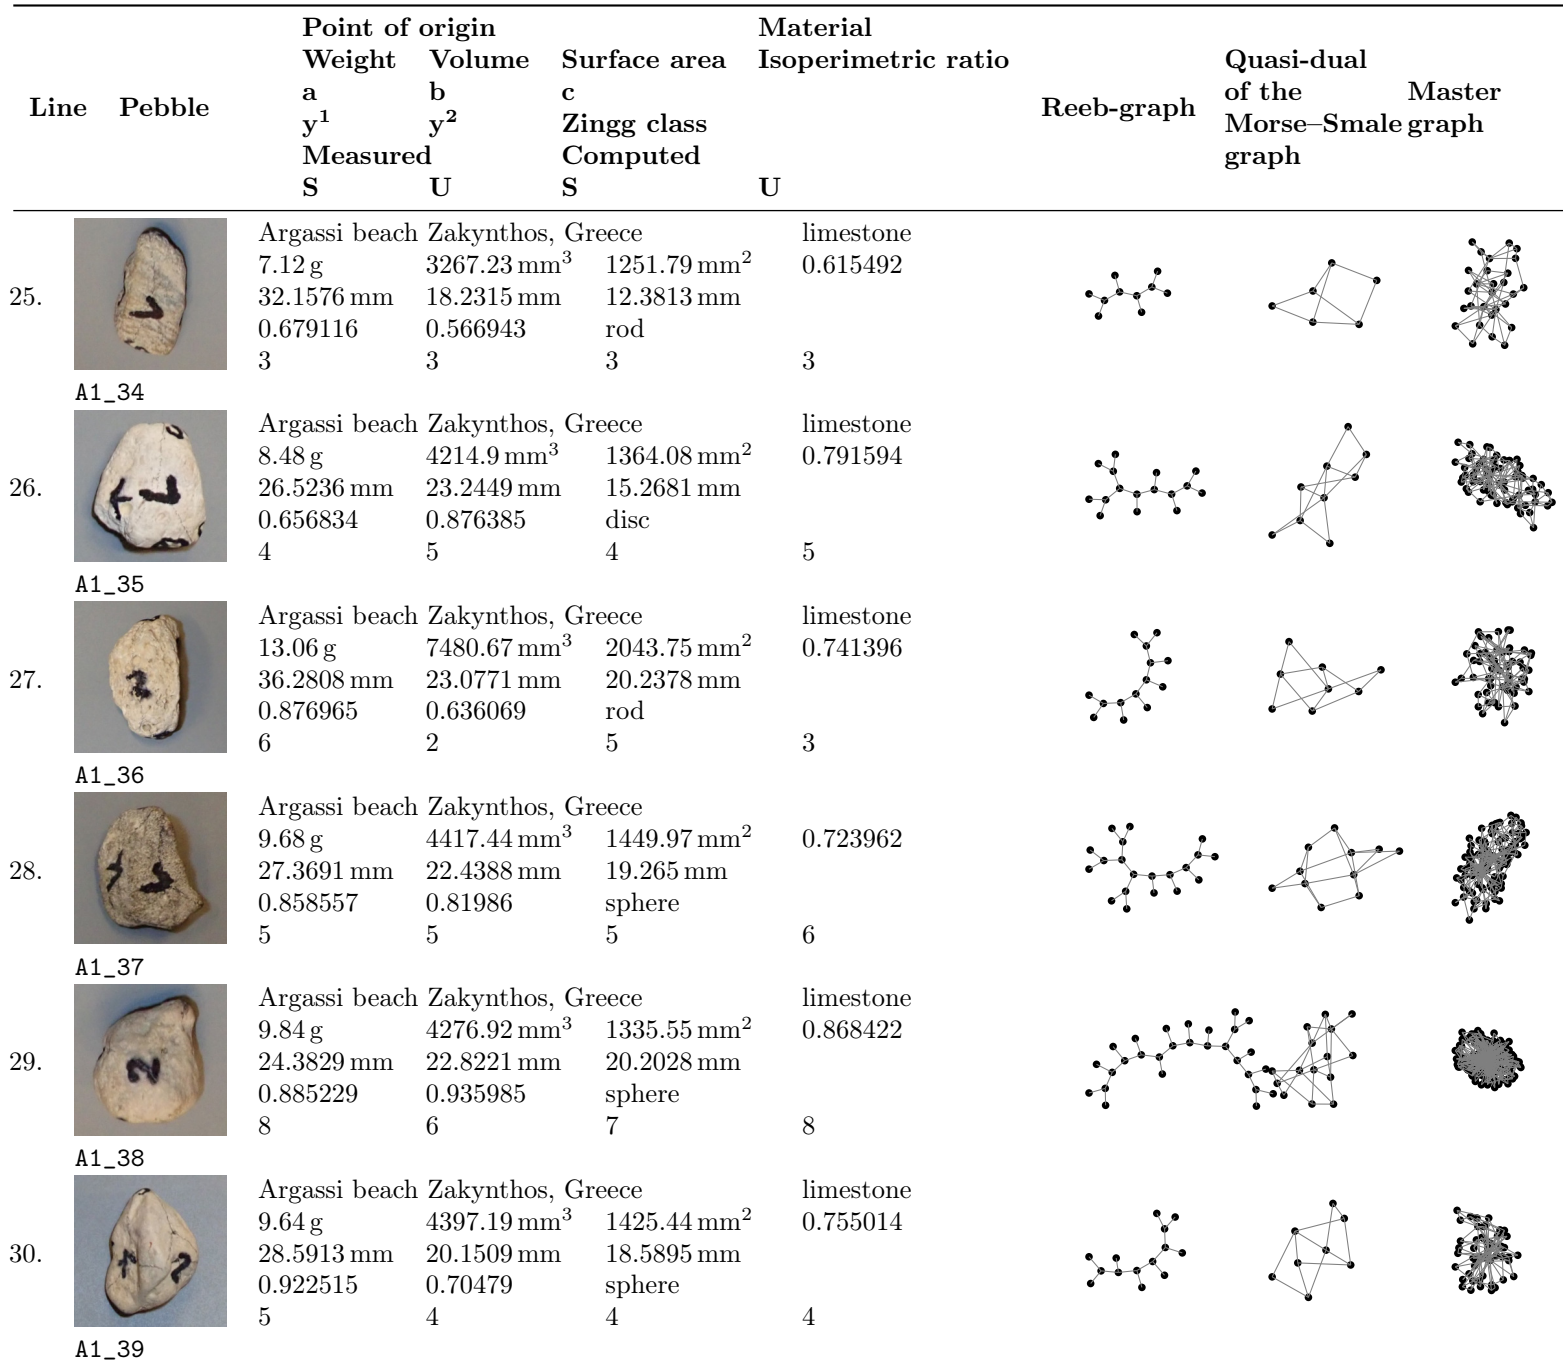 |
|      | A1_39                                                                               |                                                         |                                                                             |                                                                   |          |                                                                                       |                                                                                       |                                                                                       |

| Line | Pebble                                                                              | Point of origin                                                          |                                                        | Surface area<br>c<br>Zingg class<br>Computed<br>S    | Material<br>Isoperimetric ratio<br>U | Reeb-graph                                                                            | Quasi-dual<br>of the<br>Morse–Smale<br>graph                                          | Master<br>graph                                                                       |
|------|-------------------------------------------------------------------------------------|--------------------------------------------------------------------------|--------------------------------------------------------|------------------------------------------------------|--------------------------------------|---------------------------------------------------------------------------------------|---------------------------------------------------------------------------------------|---------------------------------------------------------------------------------------|
|      |                                                                                     | Weight                                                                   | Volume                                                 |                                                      |                                      |                                                                                       |                                                                                       |                                                                                       |
|      |                                                                                     | a<br>y <sup>1</sup><br>Measured<br>S                                     | b<br>y <sup>2</sup><br>U                               |                                                      |                                      |                                                                                       |                                                                                       |                                                                                       |
|      |                                                                                     |                                                                          |                                                        |                                                      |                                      |                                                                                       |                                                                                       |                                                                                       |
| 31.  | 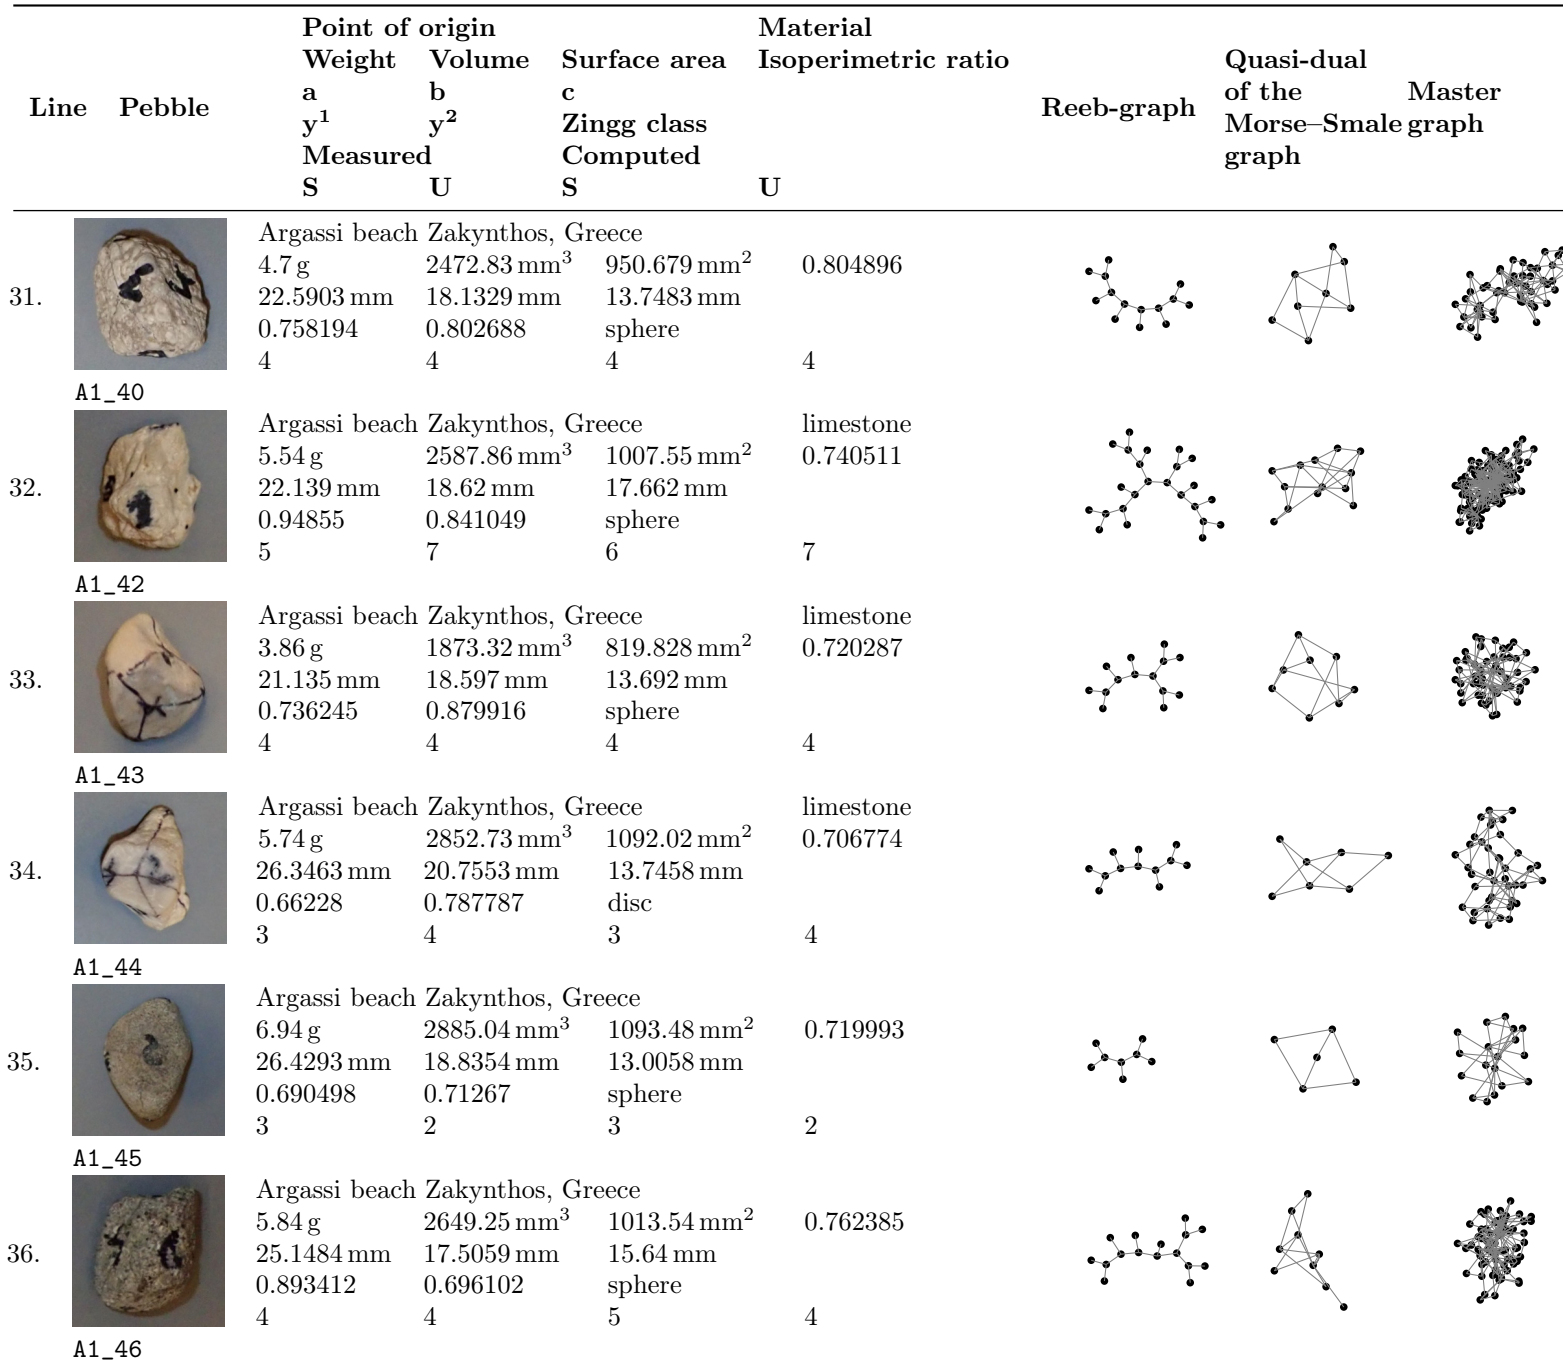   | Argassi beach Zakynthos, Greece<br>4.7 g<br>22.5903 mm<br>0.758194<br>4  | 2472.83 mm <sup>3</sup><br>18.1329 mm<br>0.802688<br>4 | 950.679 mm <sup>2</sup><br>13.7483 mm<br>sphere<br>4 | 0.804896                             | 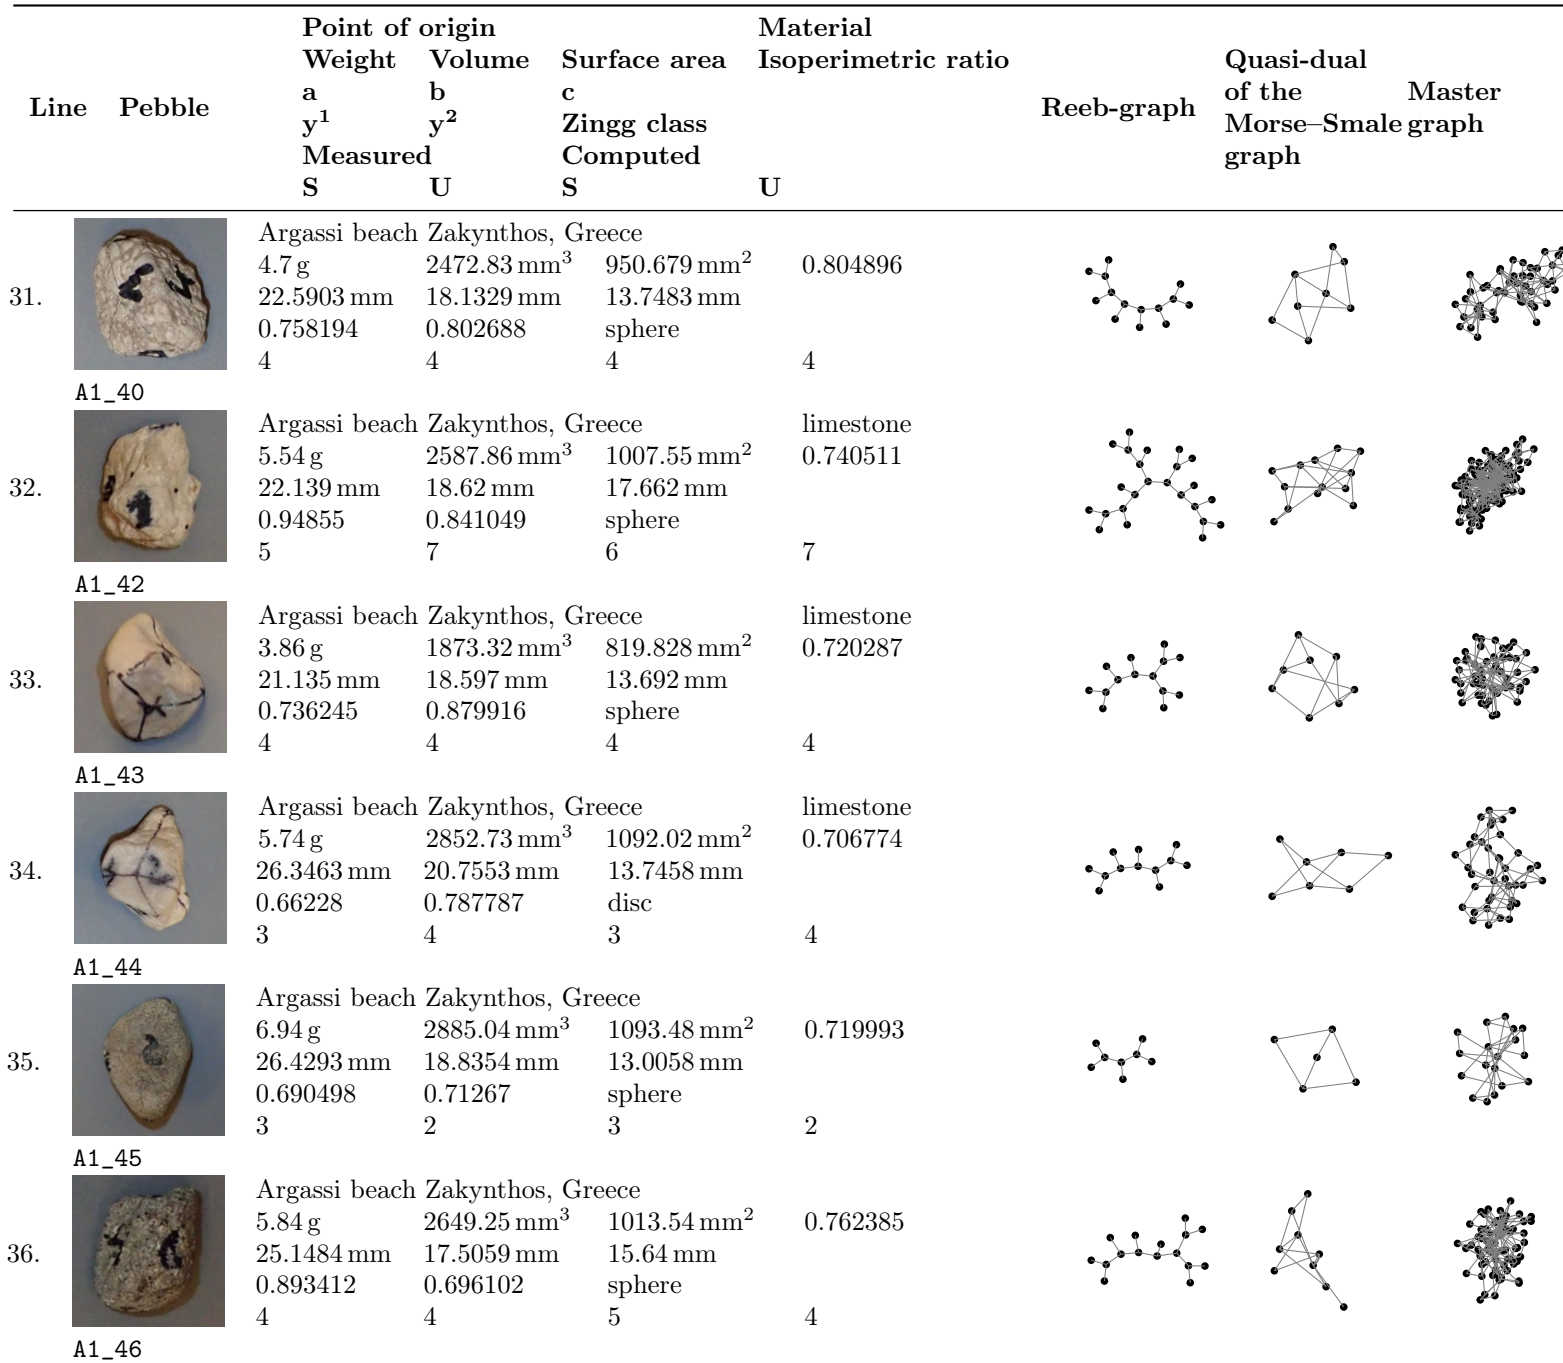   | 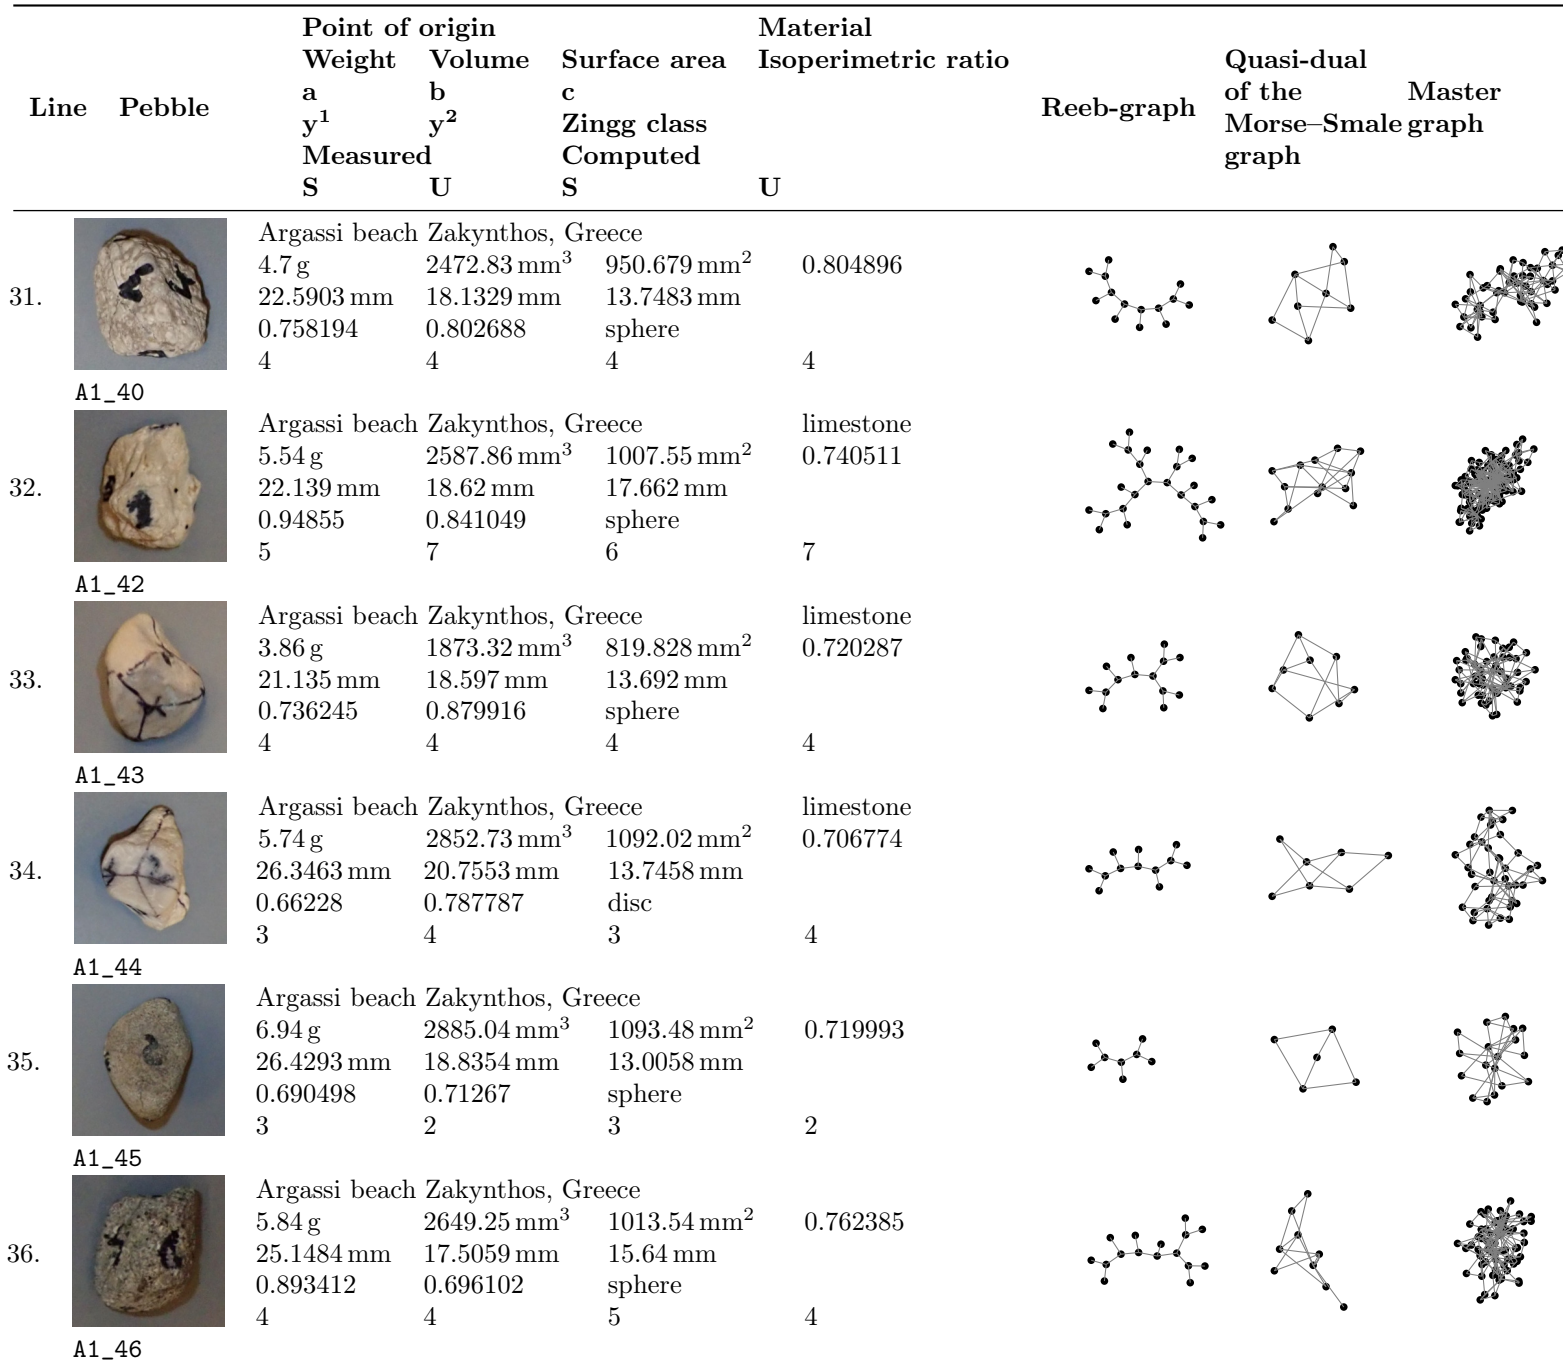   | 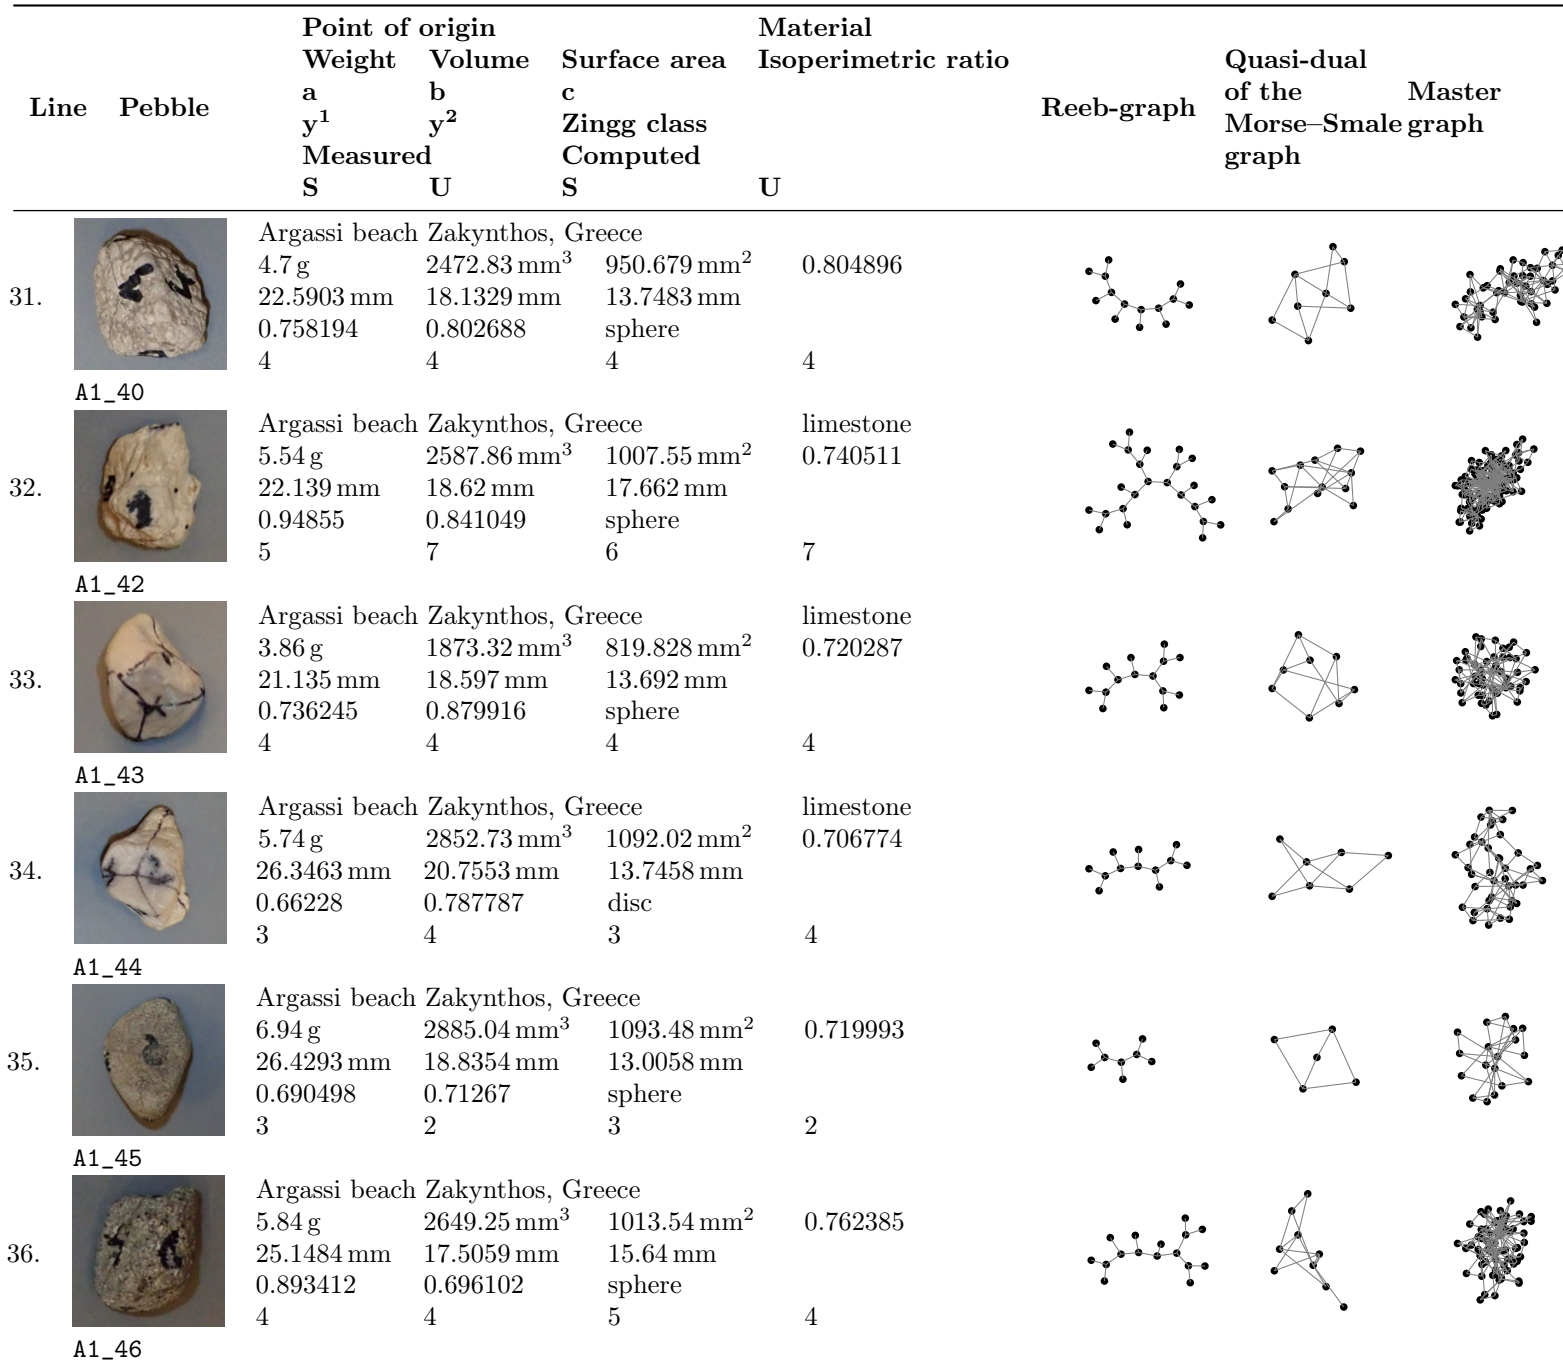   |
|      | A1_40                                                                               |                                                                          |                                                        |                                                      |                                      |                                                                                       |                                                                                       |                                                                                       |
| 32.  | 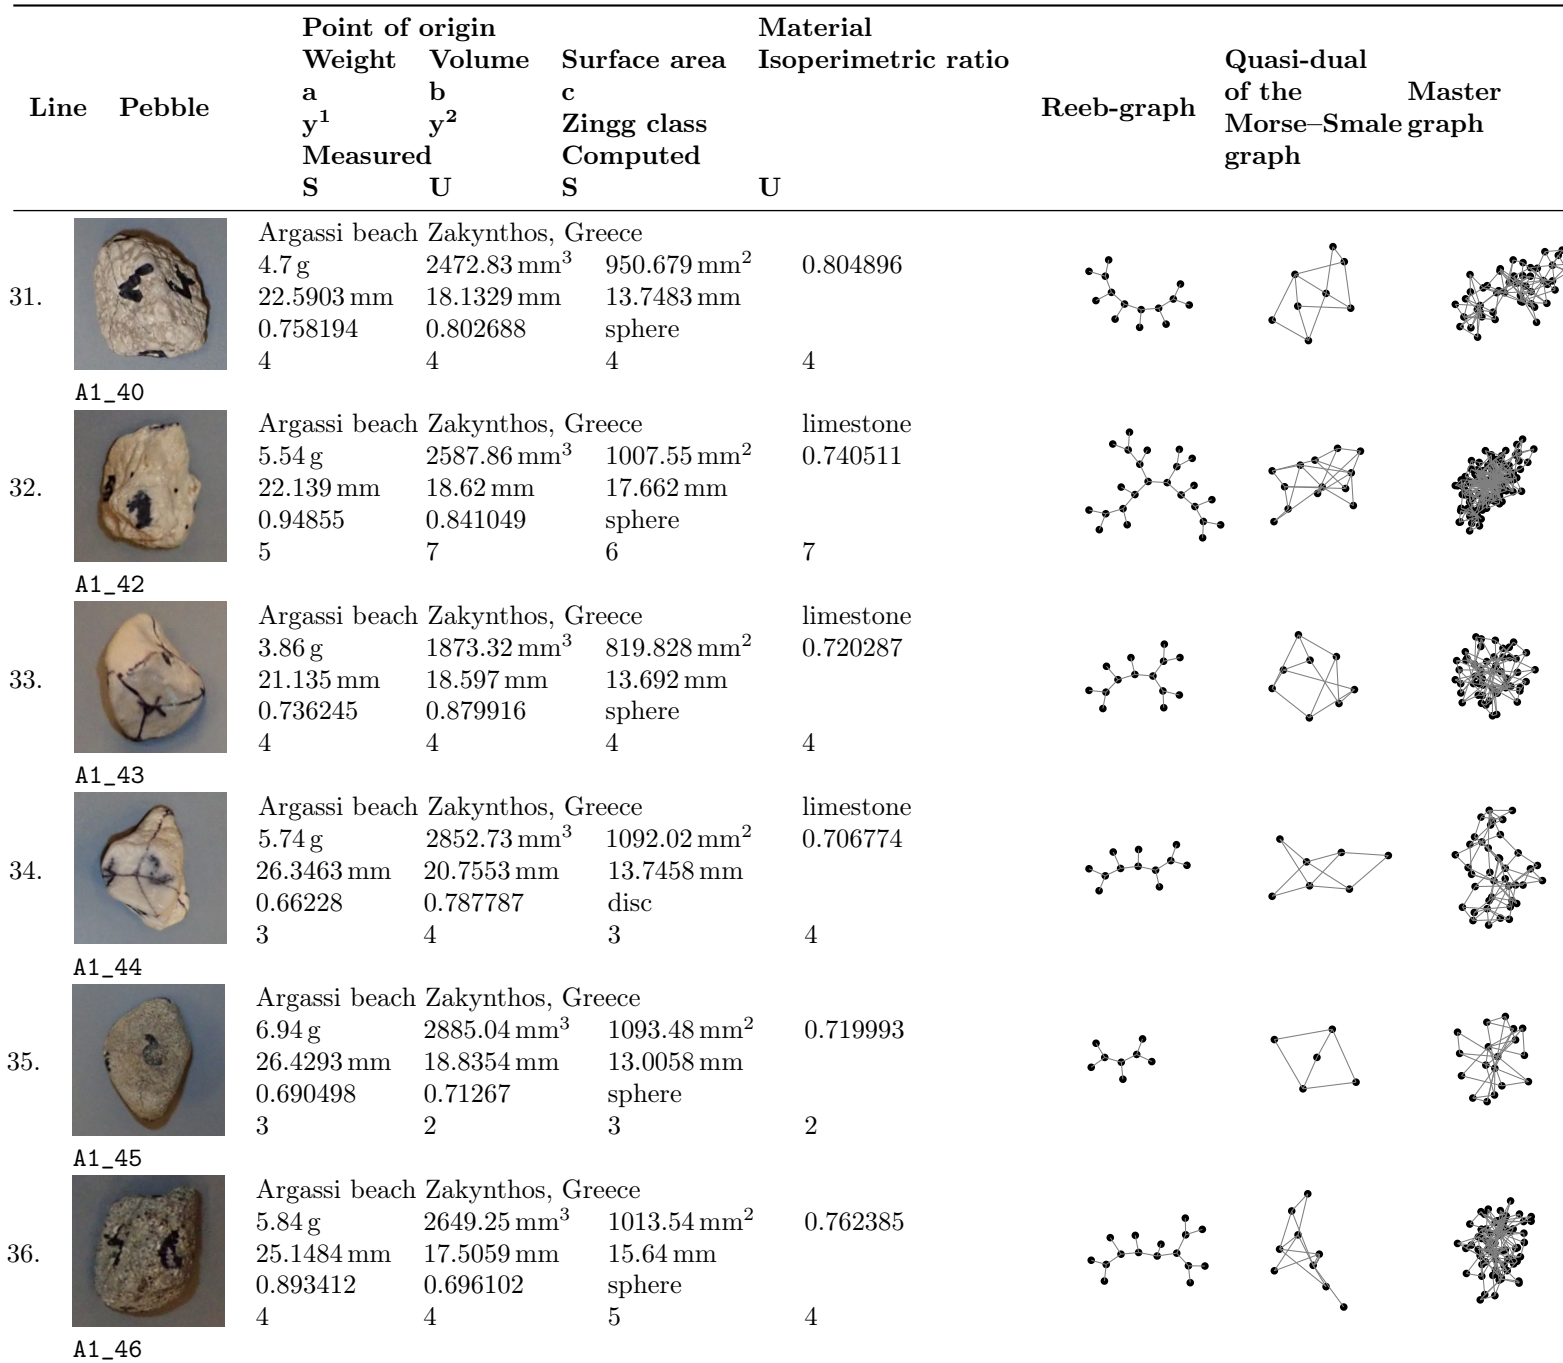   | Argassi beach Zakynthos, Greece<br>5.54 g<br>22.139 mm<br>0.94855<br>5   | 2587.86 mm <sup>3</sup><br>18.62 mm<br>0.841049<br>7   | 1007.55 mm <sup>2</sup><br>17.662 mm<br>sphere<br>6  | limestone<br>0.740511                | 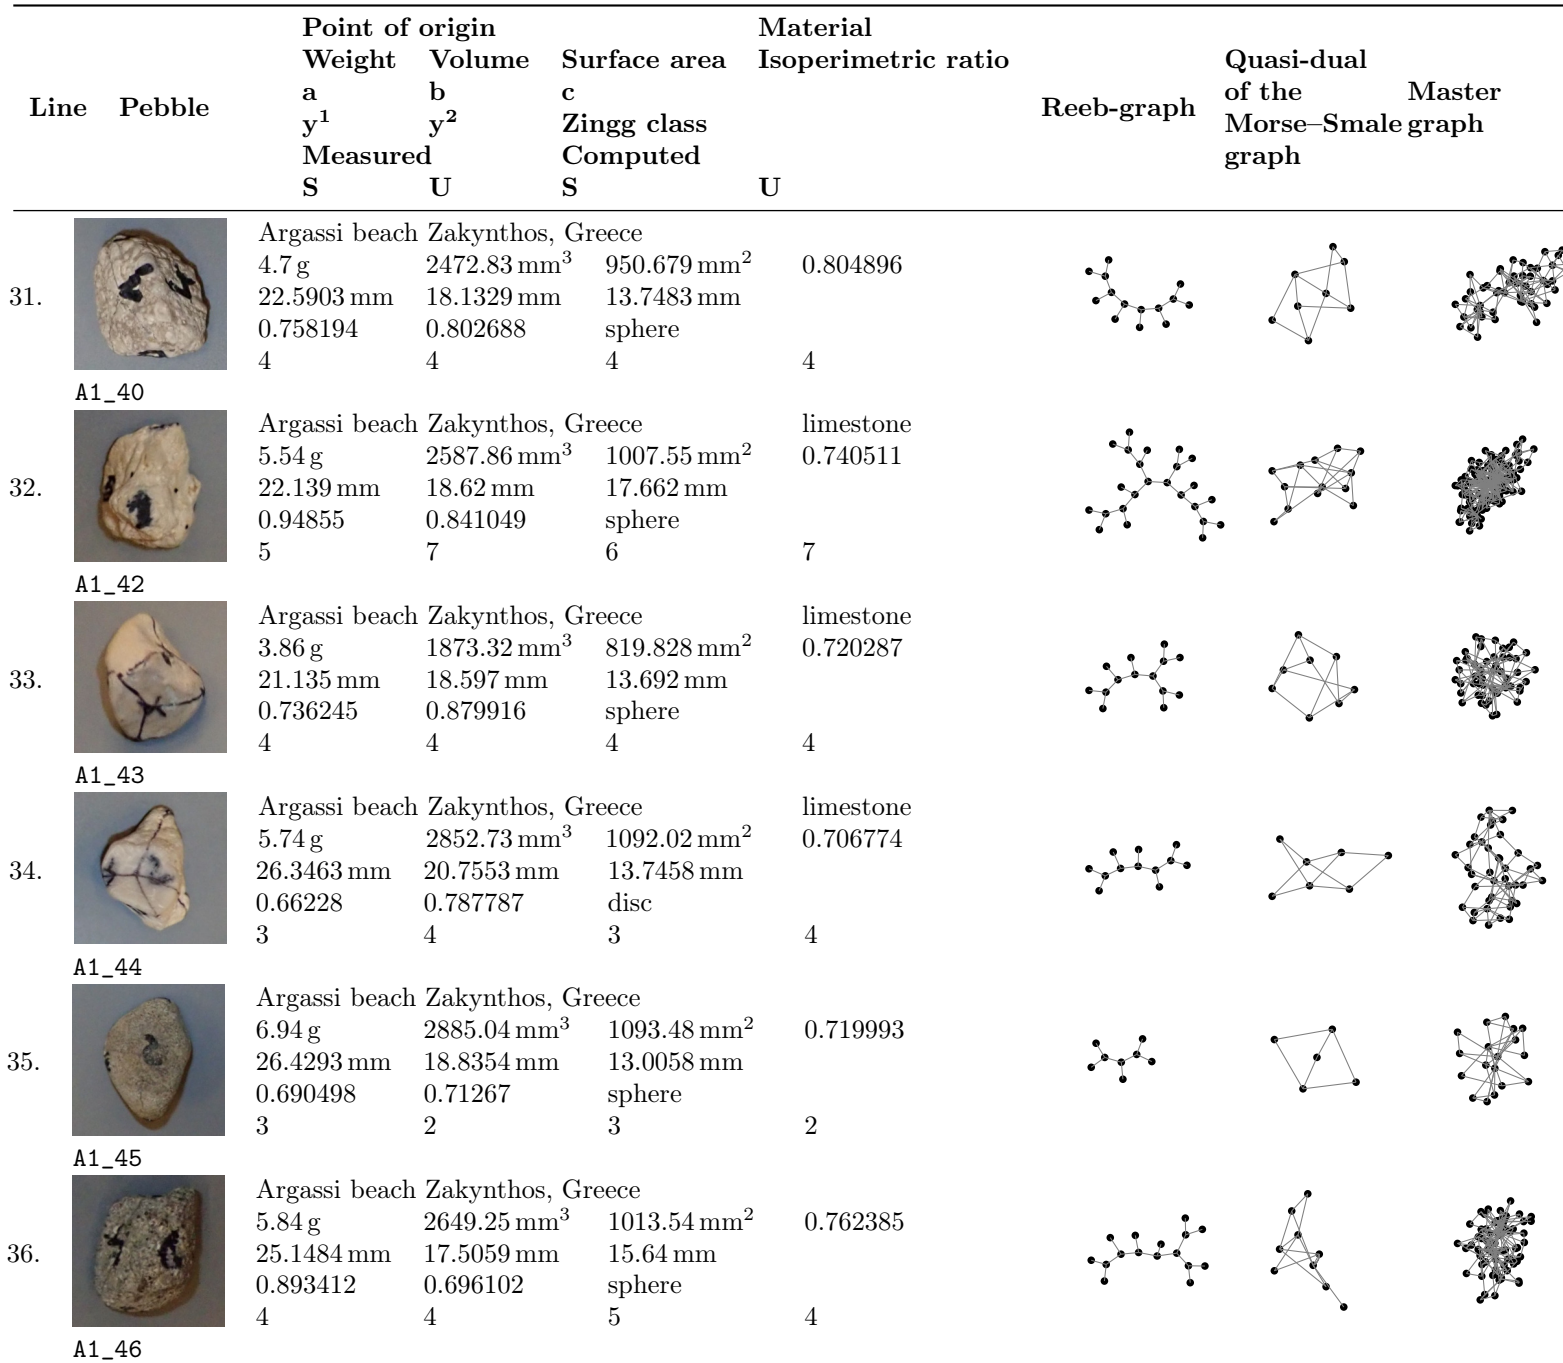   | 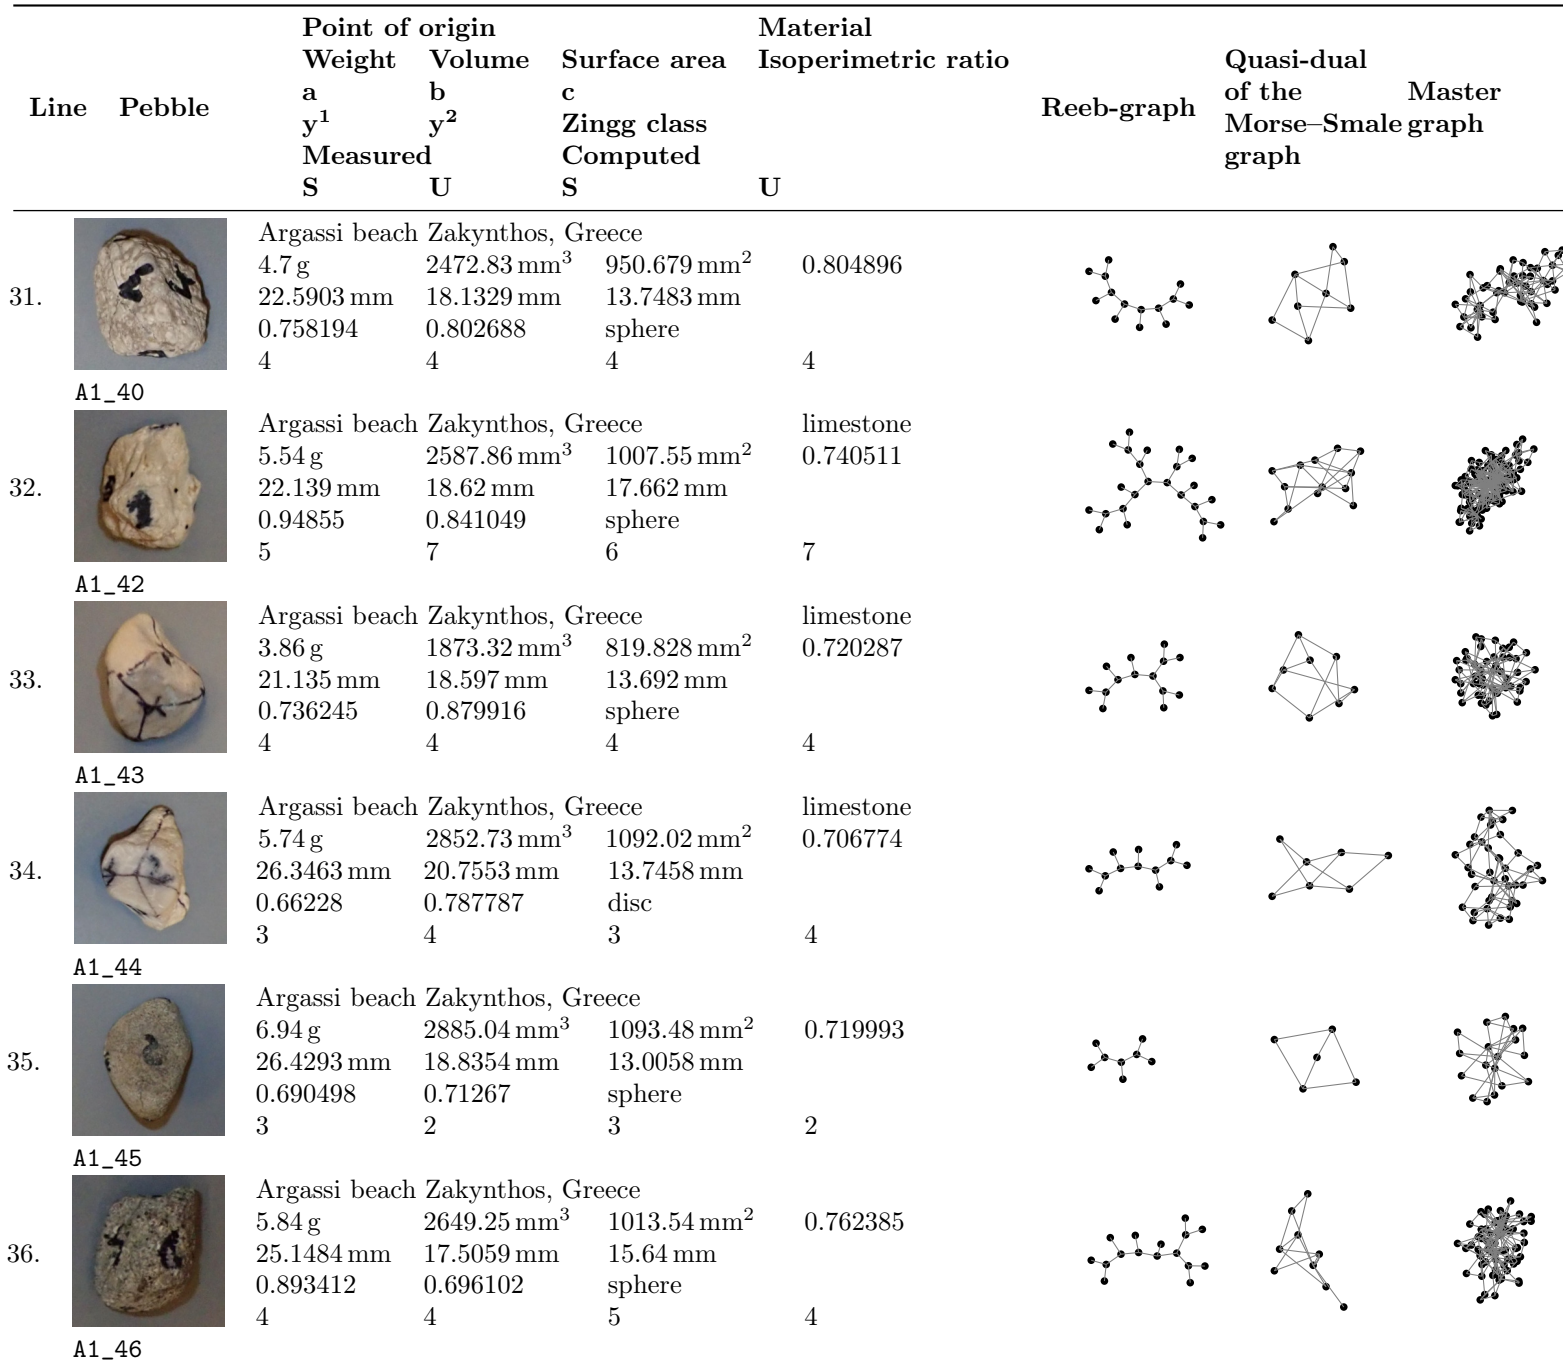   | 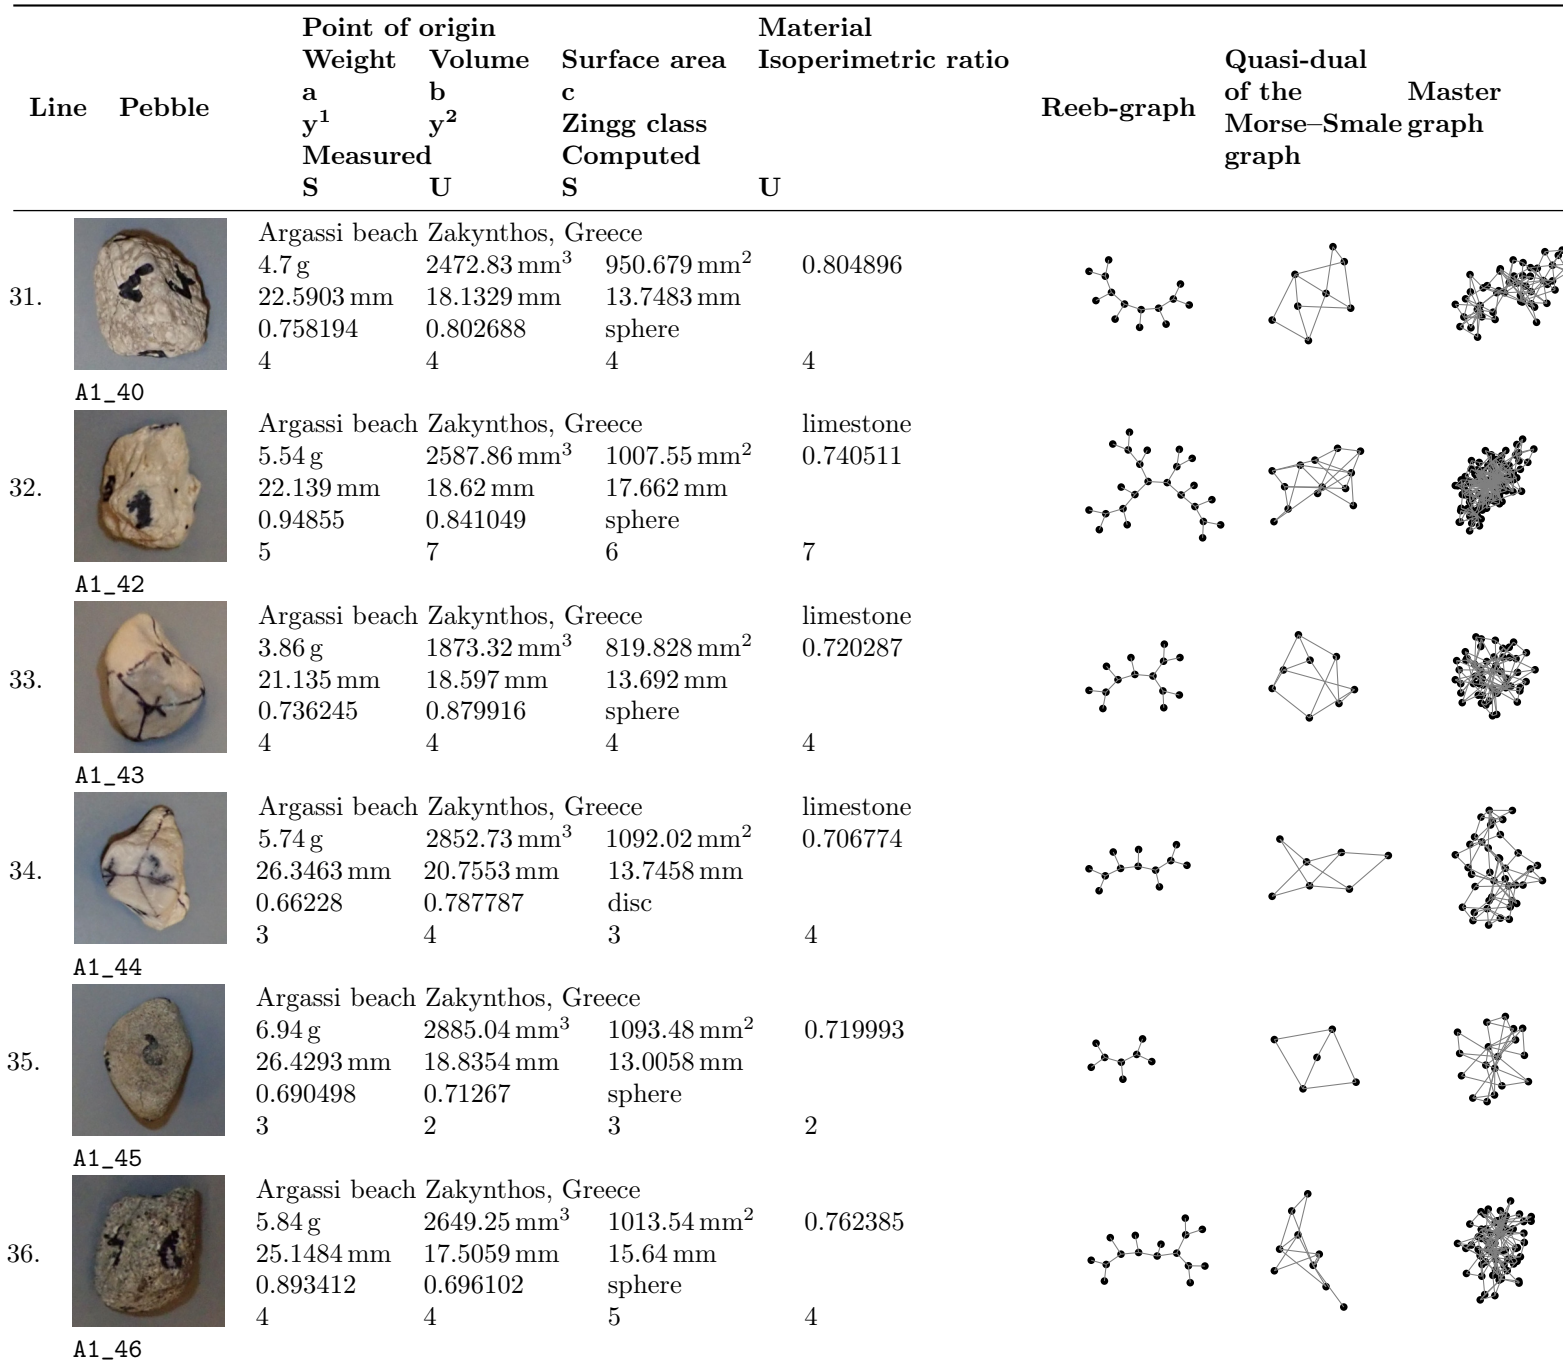   |
|      | A1_42                                                                               |                                                                          |                                                        |                                                      |                                      |                                                                                       |                                                                                       |                                                                                       |
| 33.  | 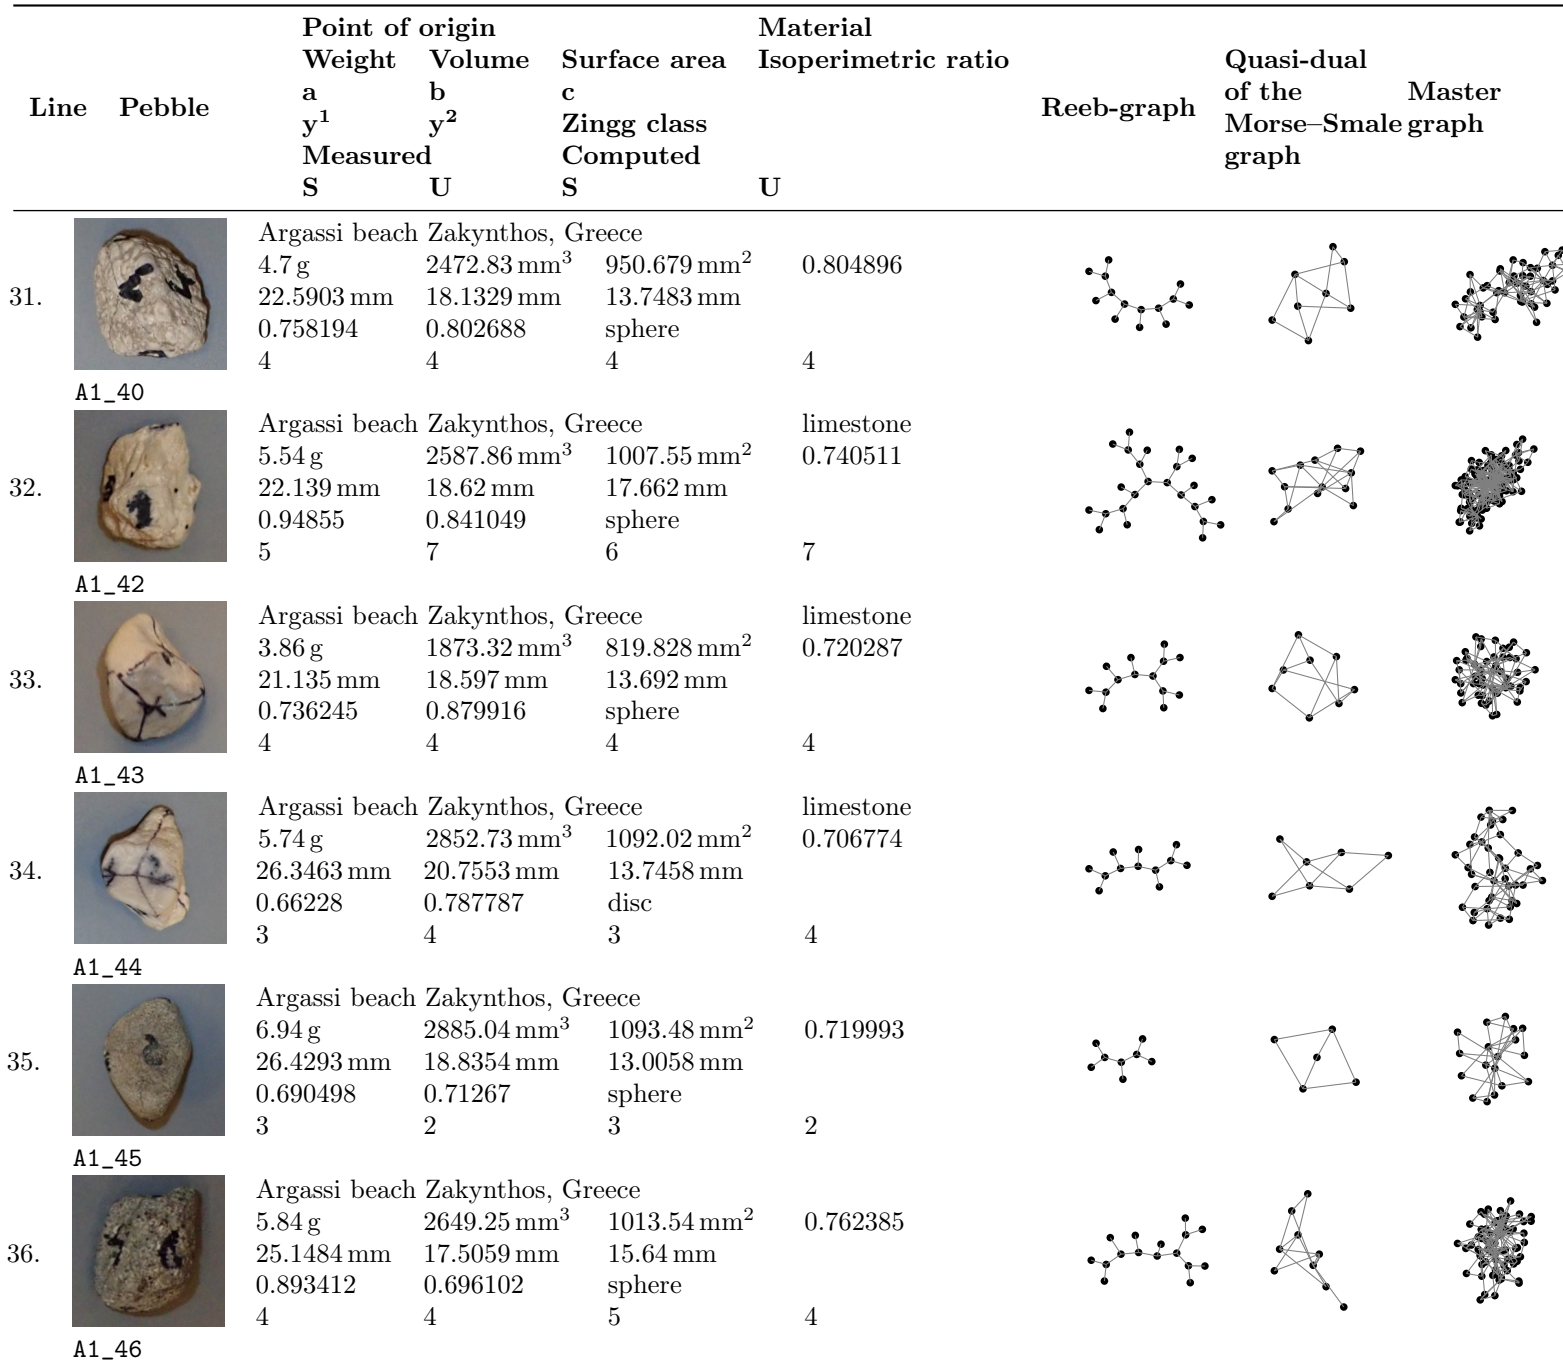   | Argassi beach Zakynthos, Greece<br>3.86 g<br>21.135 mm<br>0.736245<br>4  | 1873.32 mm <sup>3</sup><br>18.597 mm<br>0.879916<br>4  | 819.828 mm <sup>2</sup><br>13.692 mm<br>sphere<br>4  | limestone<br>0.720287                | 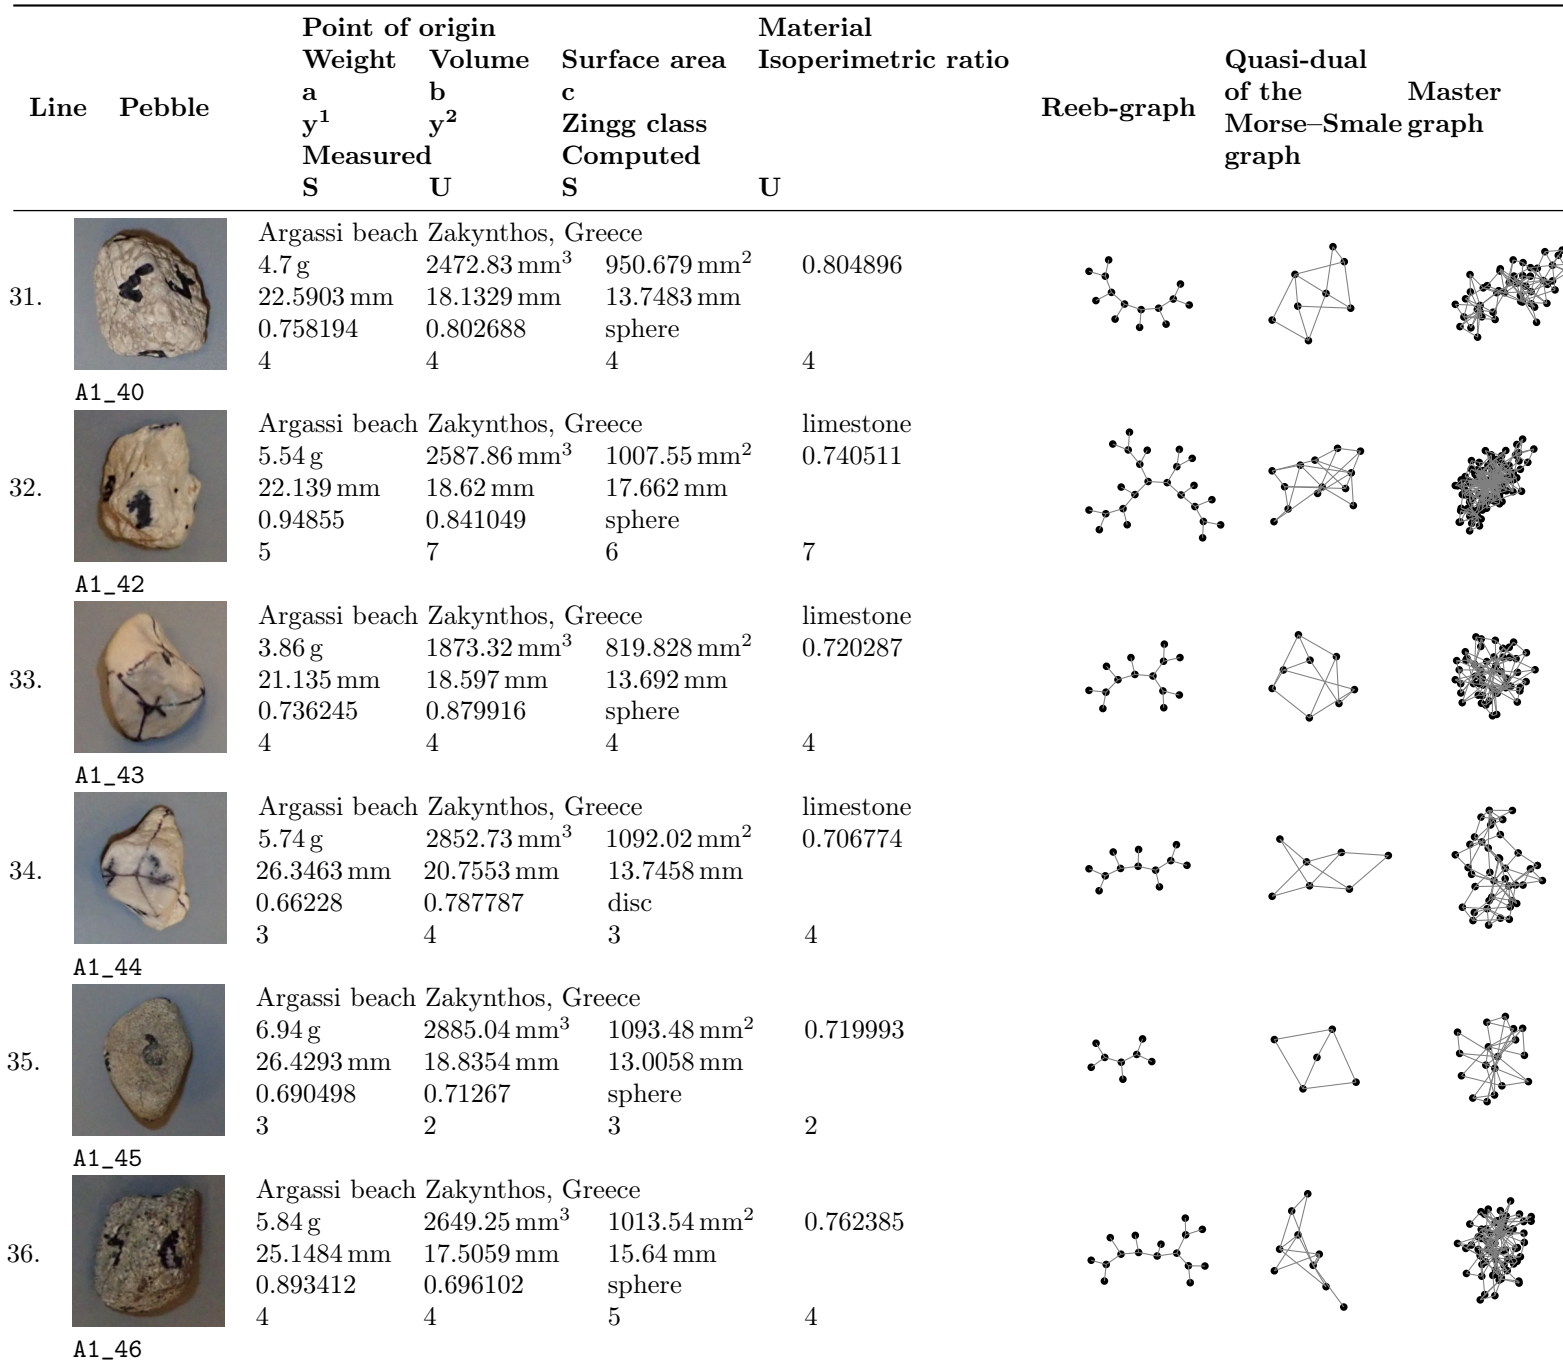   | 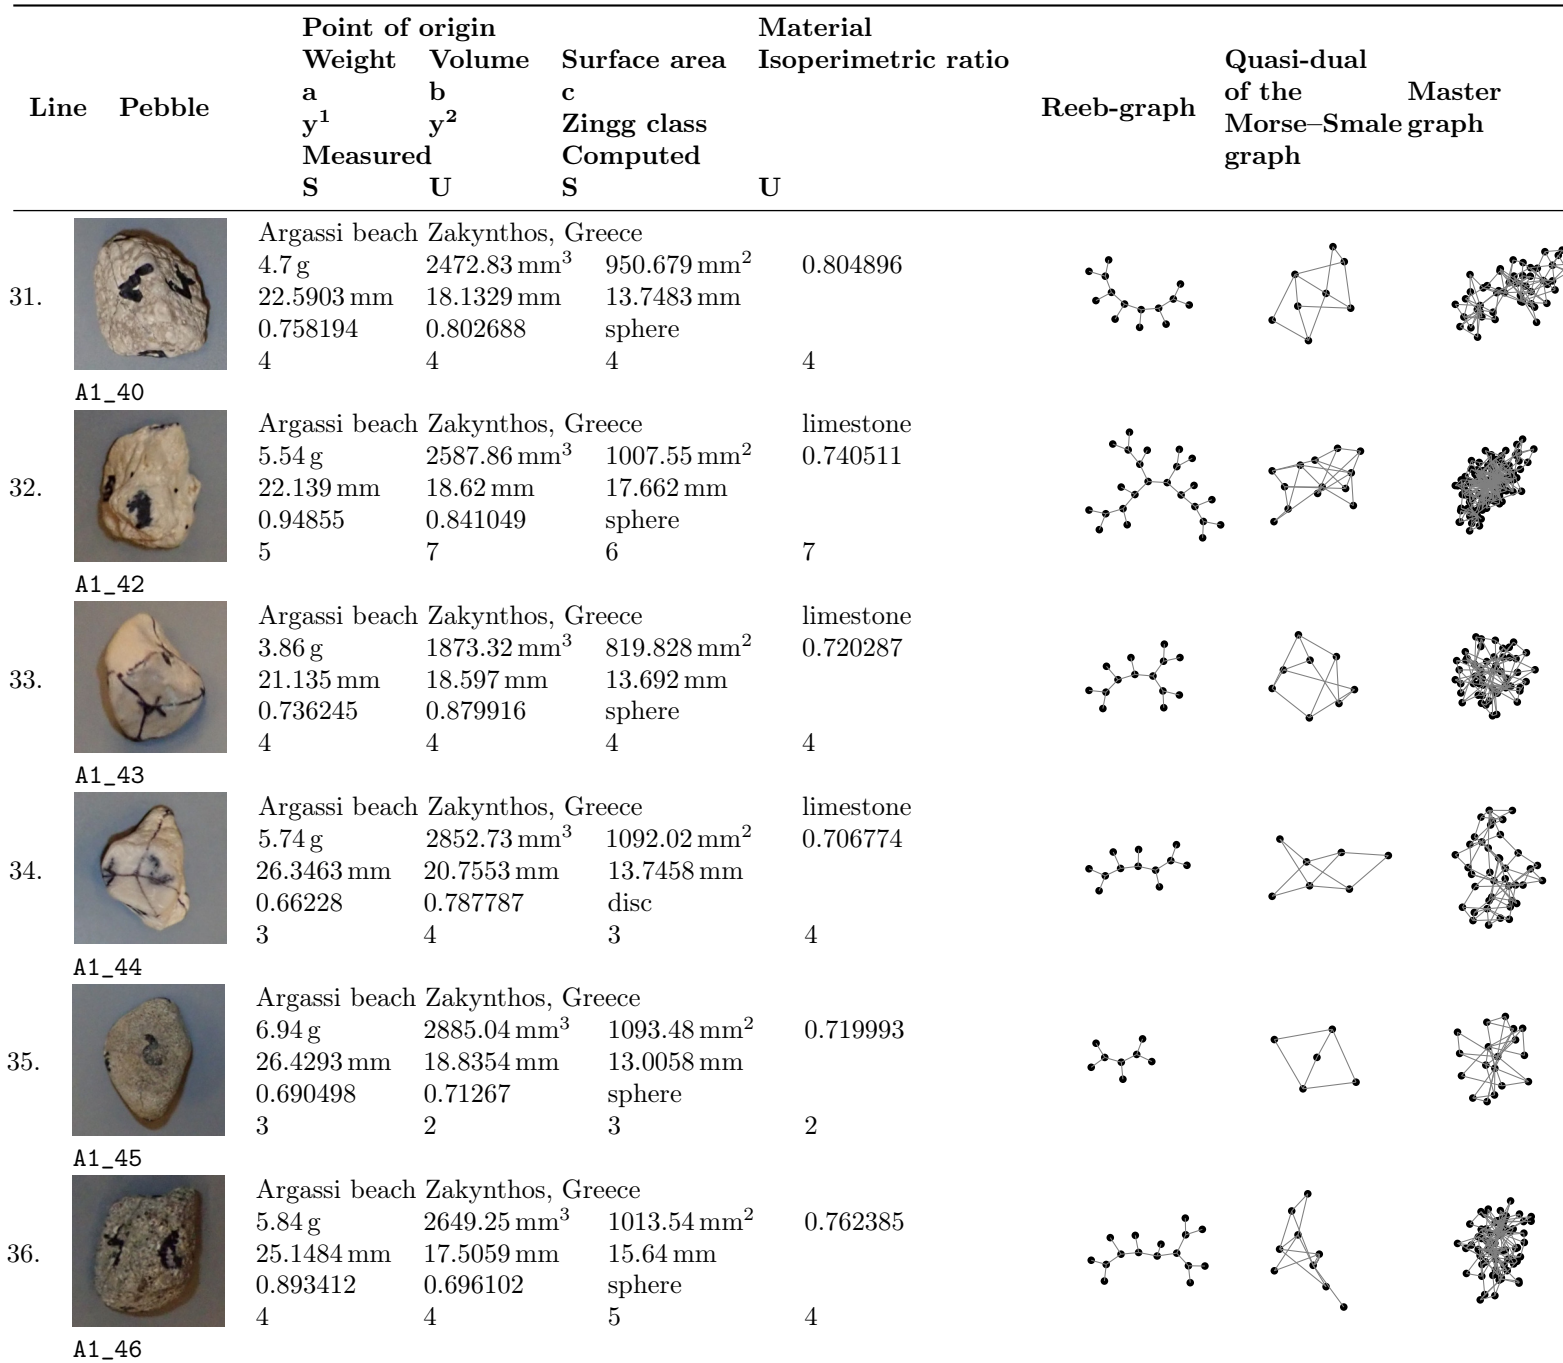   | 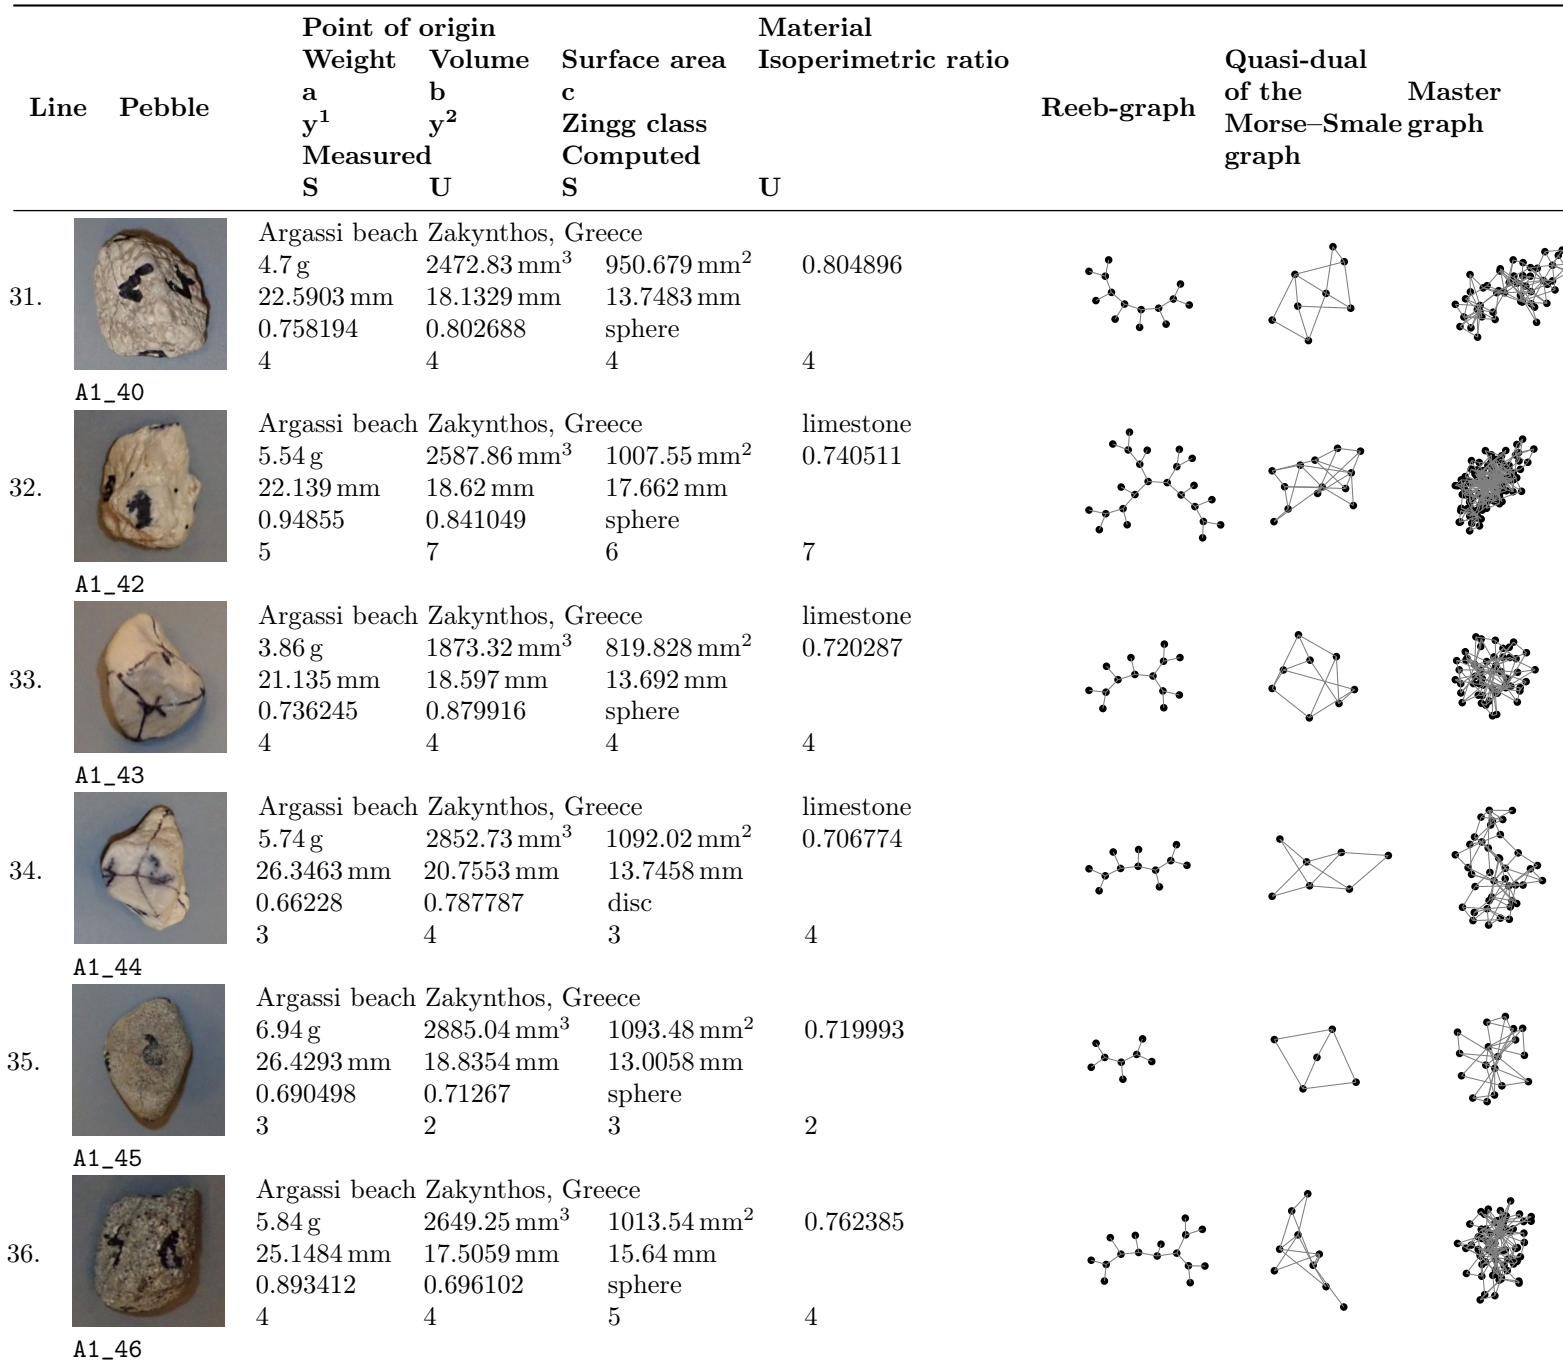   |
|      | A1_43                                                                               |                                                                          |                                                        |                                                      |                                      |                                                                                       |                                                                                       |                                                                                       |
| 34.  | 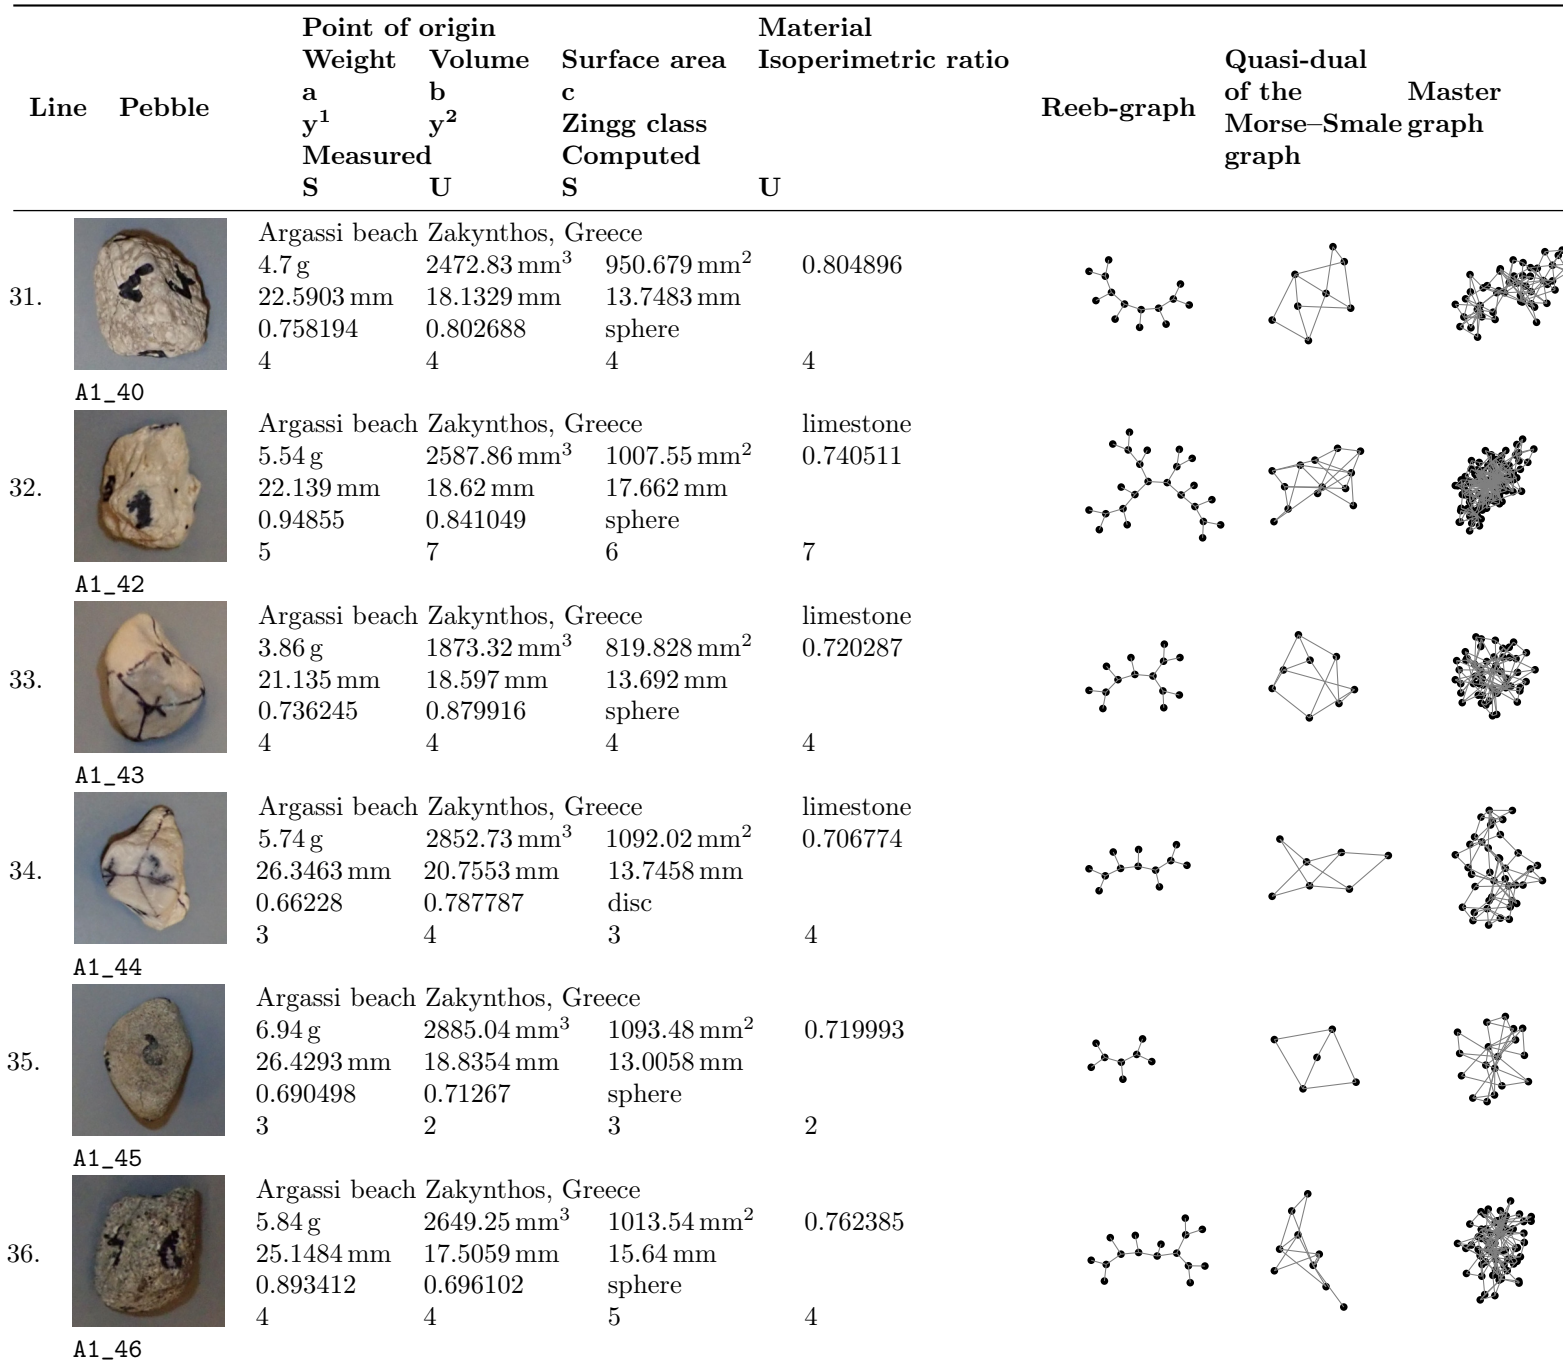  | Argassi beach Zakynthos, Greece<br>5.74 g<br>26.3463 mm<br>0.66228<br>3  | 2852.73 mm <sup>3</sup><br>20.7553 mm<br>0.787787<br>4 | 1092.02 mm <sup>2</sup><br>13.7458 mm<br>disc<br>3   | limestone<br>0.706774                | 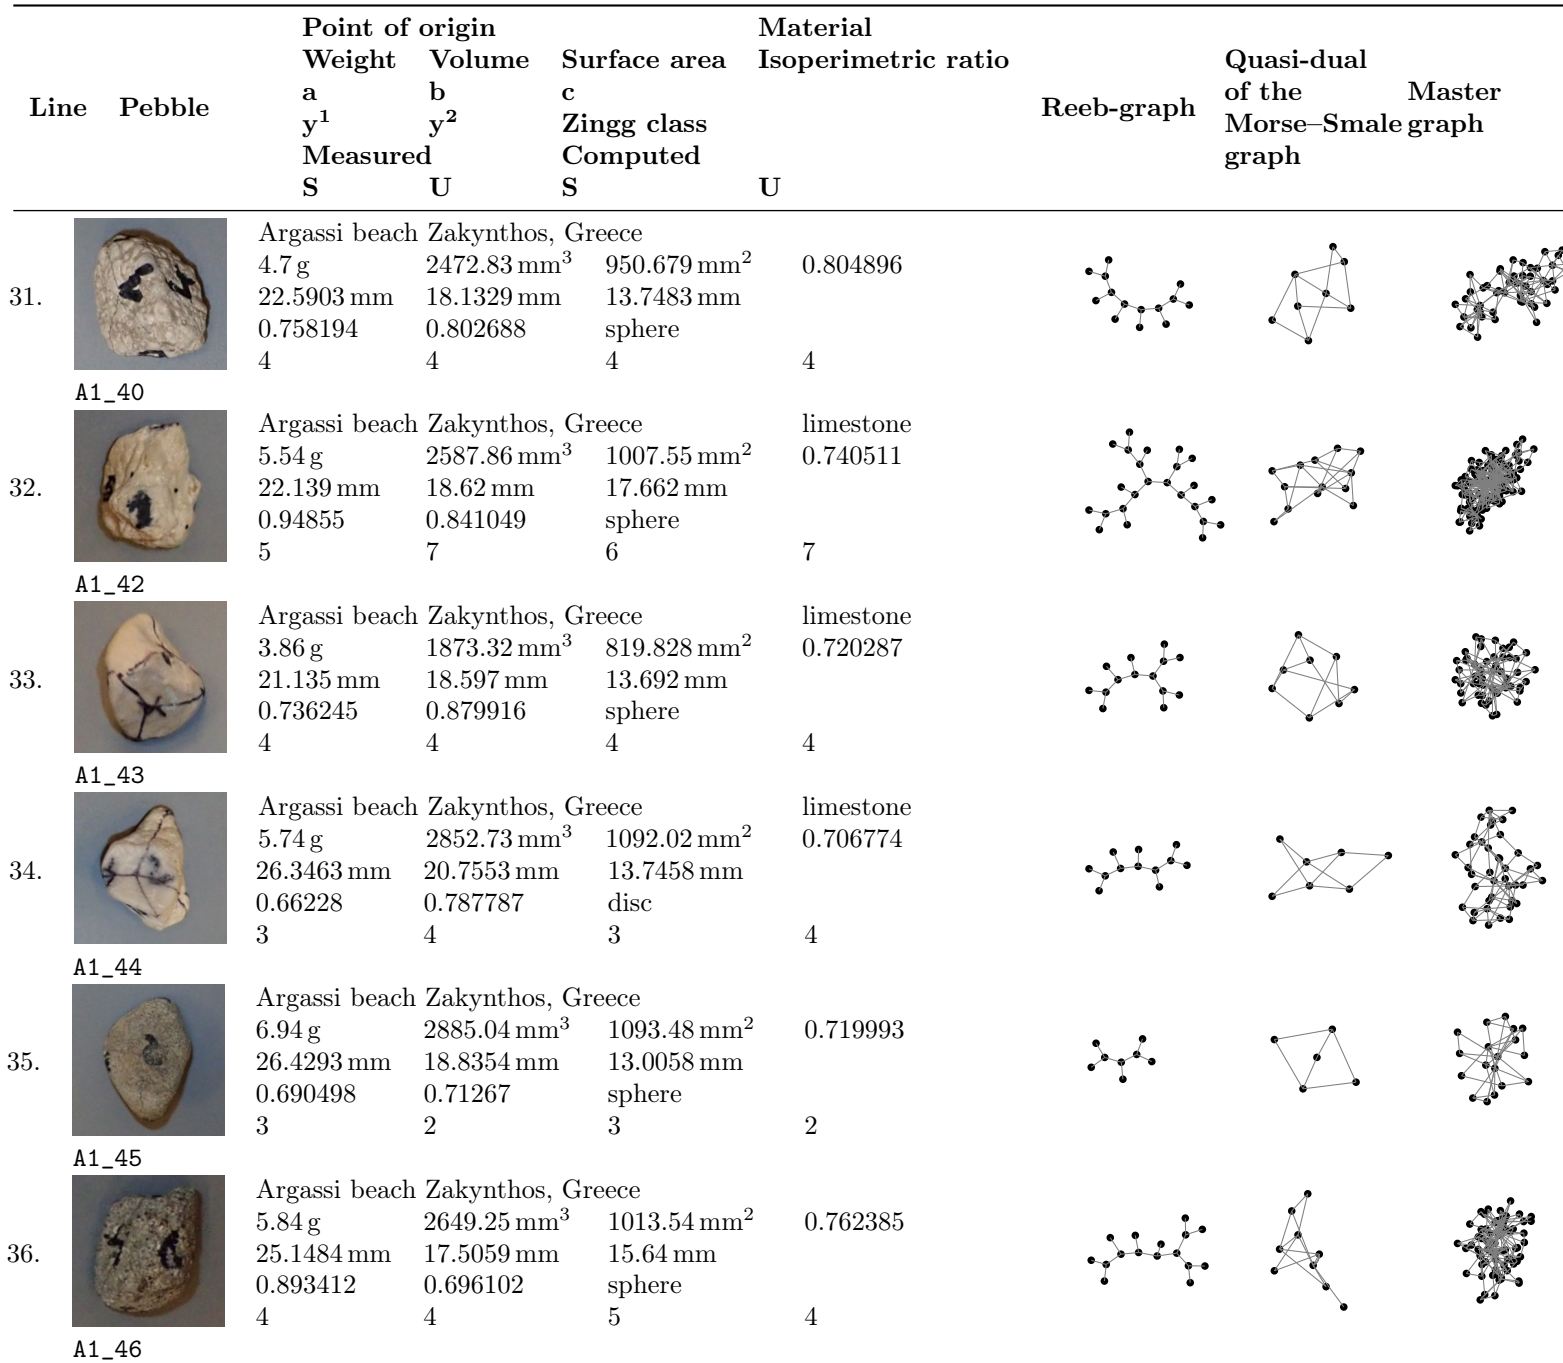  | 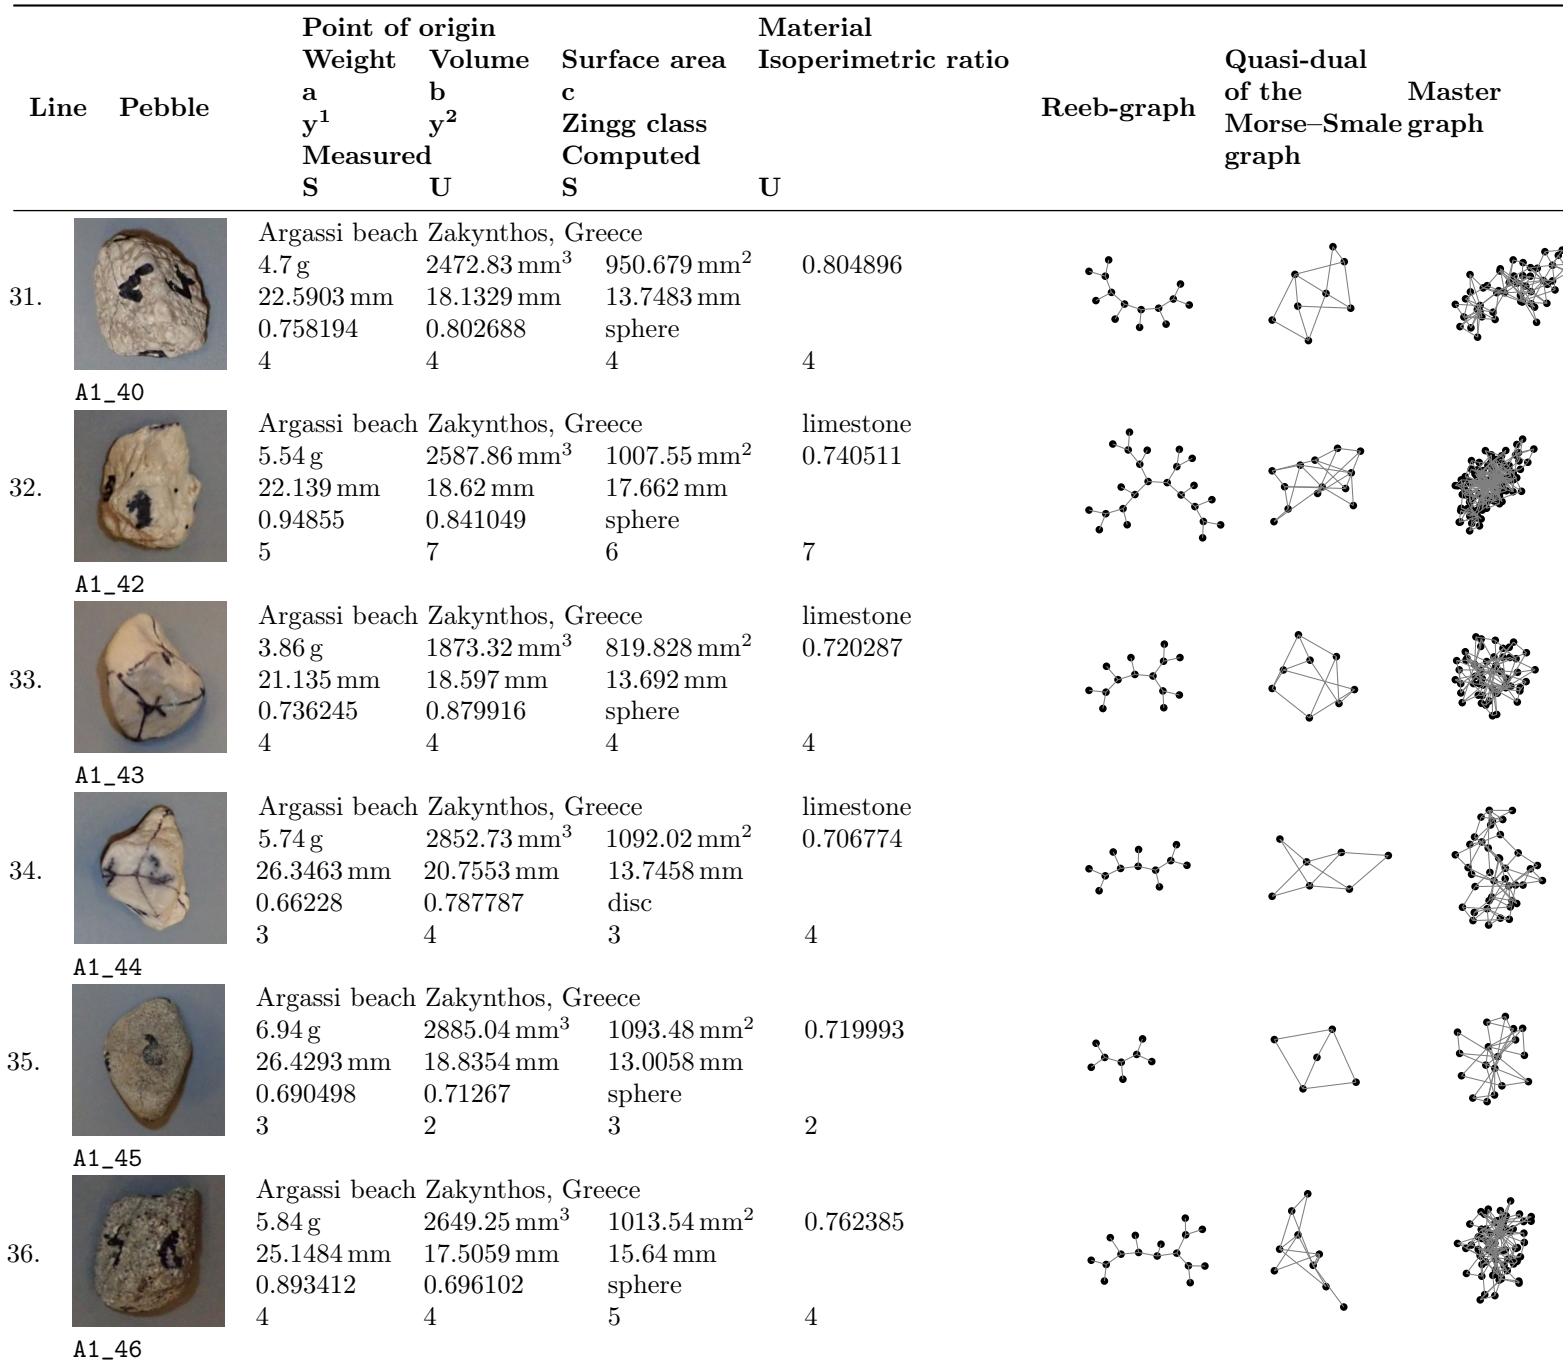  | 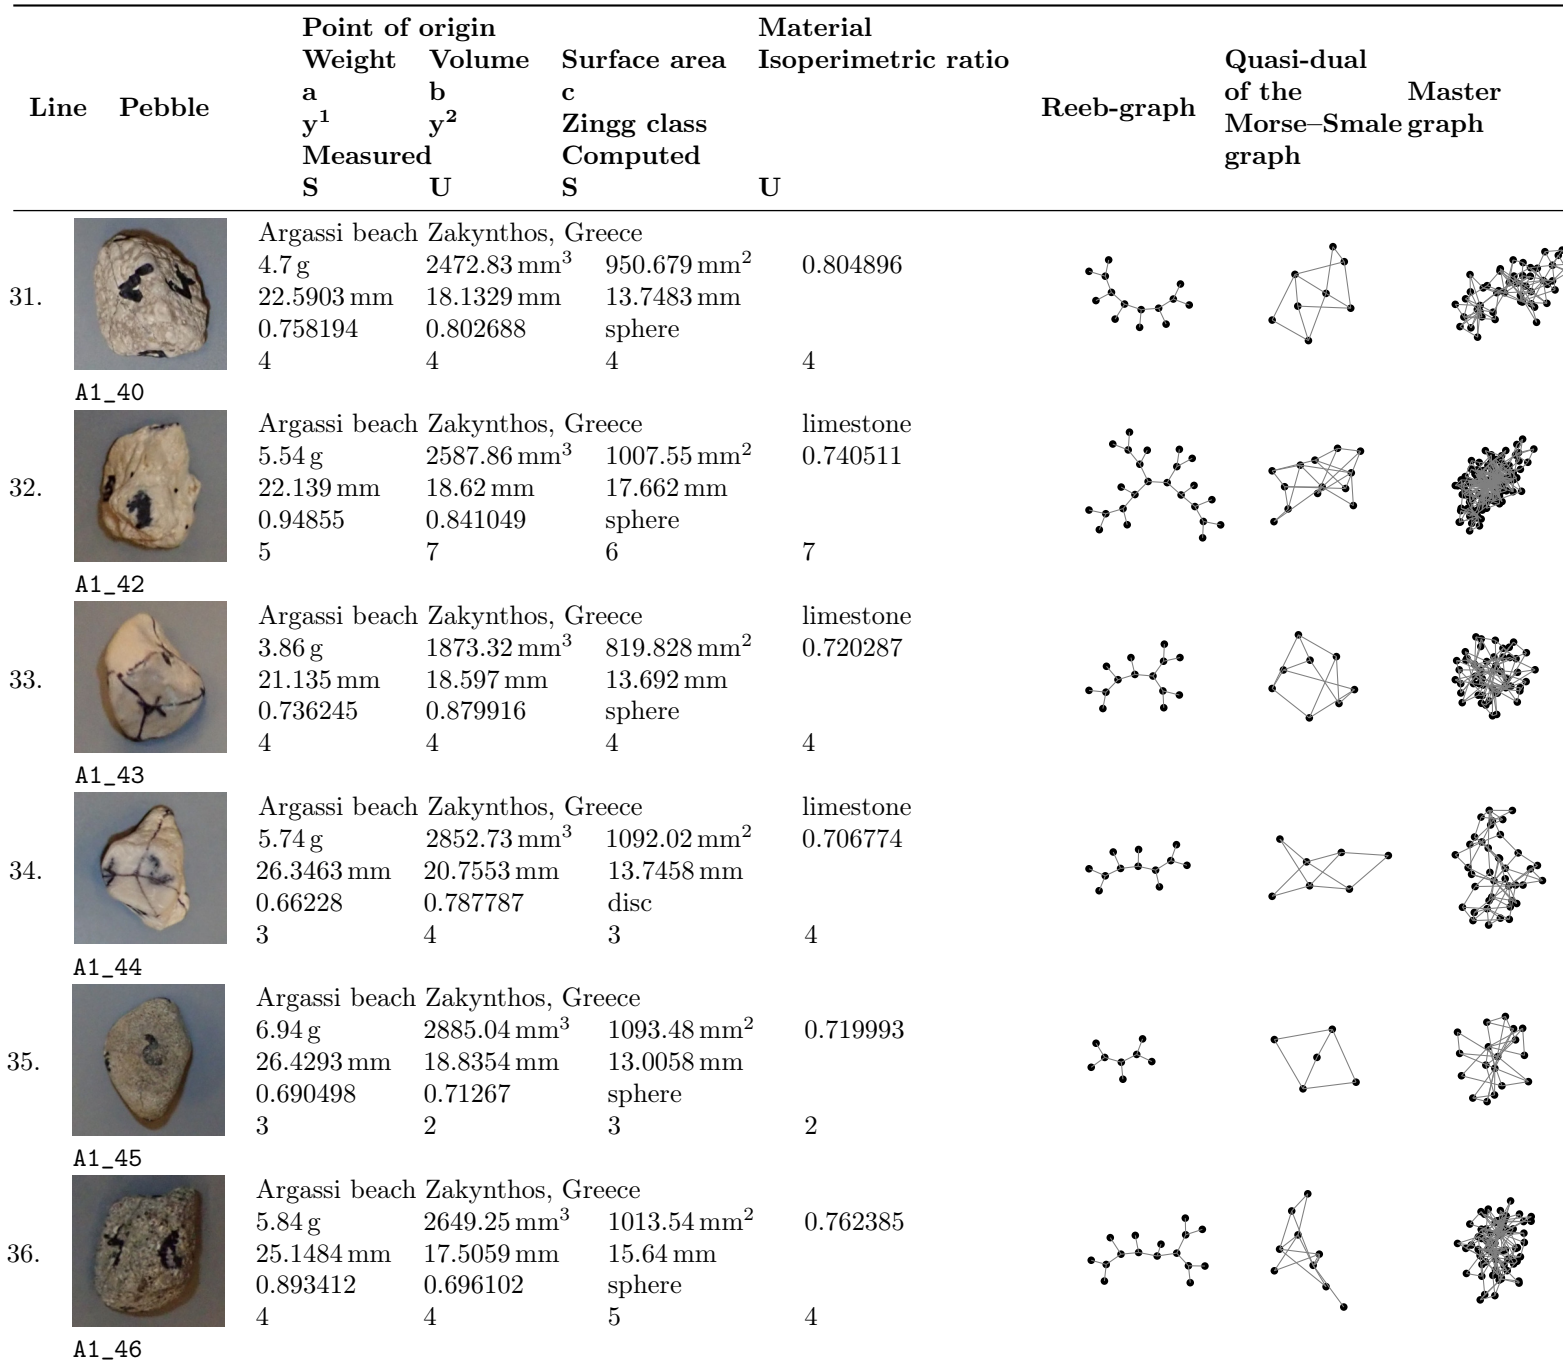  |
|      | A1_44                                                                               |                                                                          |                                                        |                                                      |                                      |                                                                                       |                                                                                       |                                                                                       |
| 35.  | 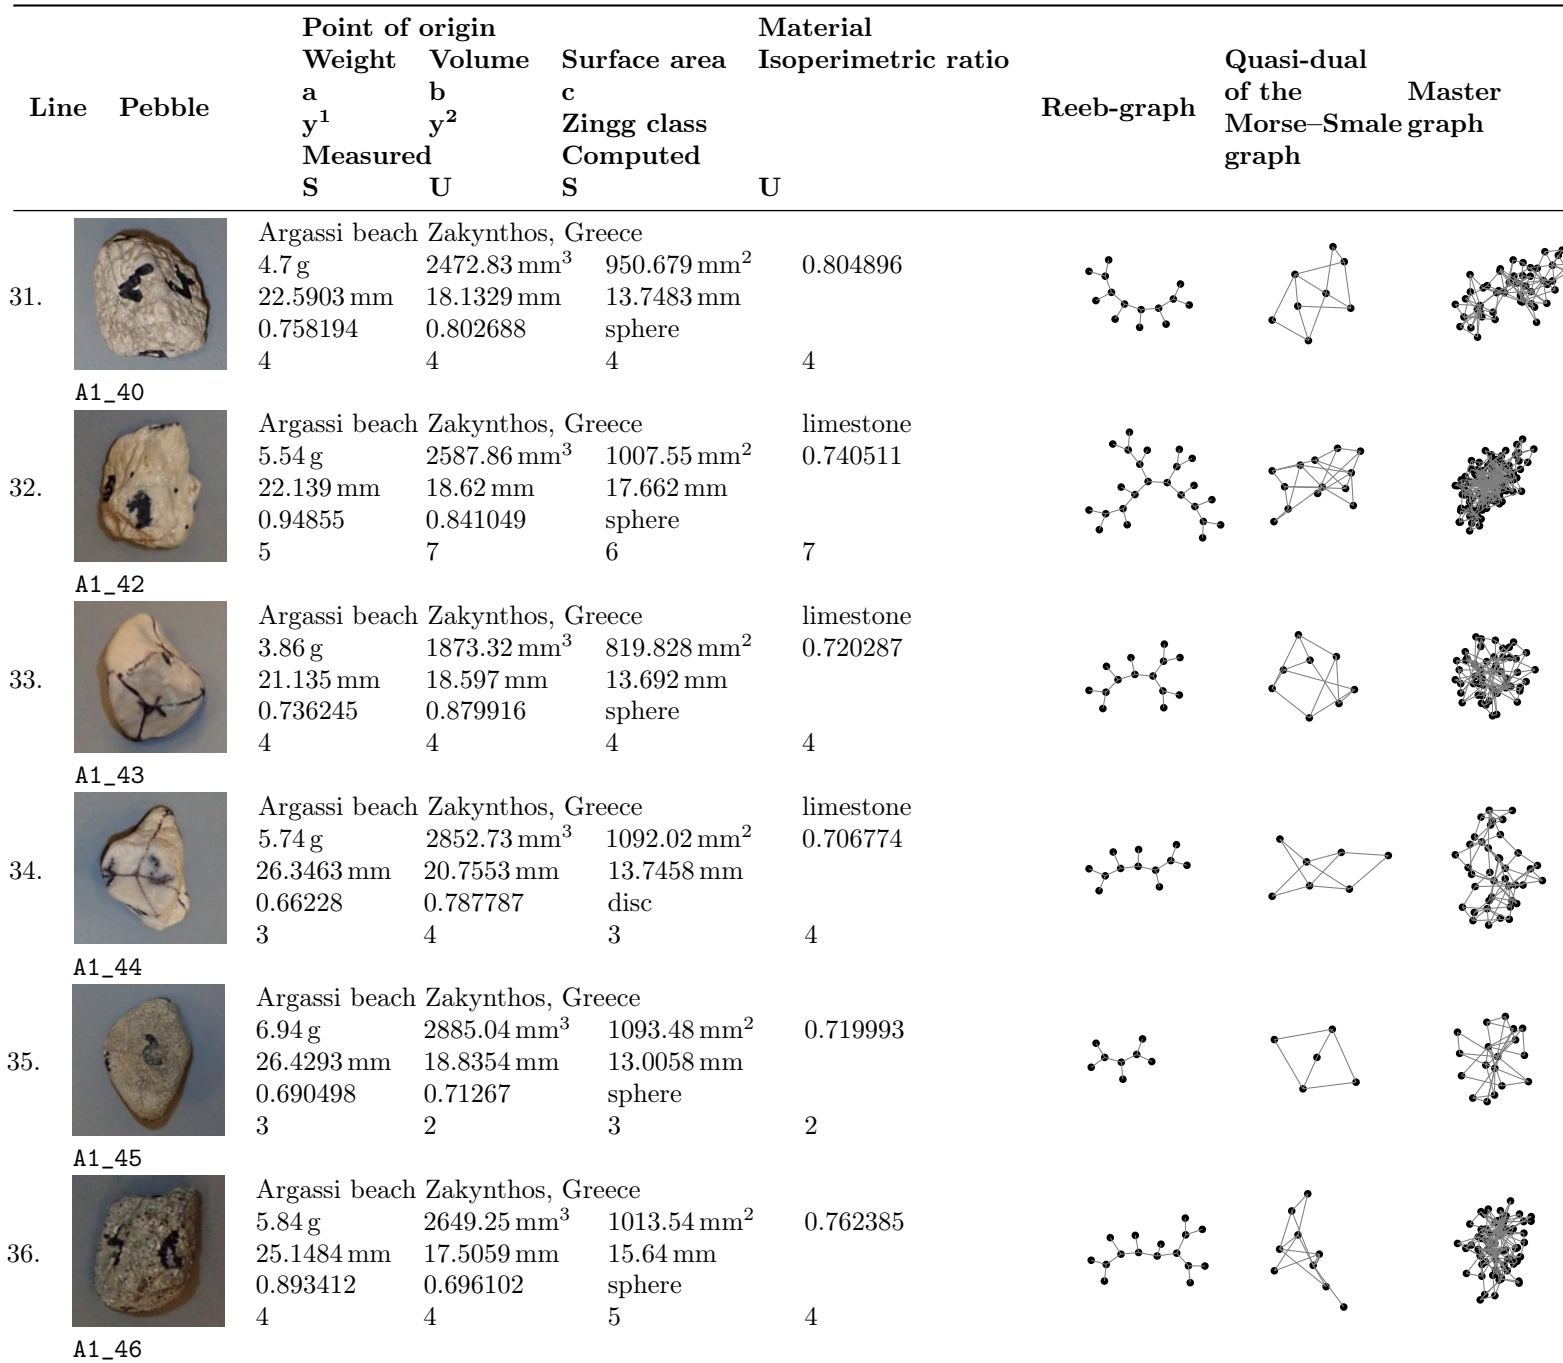 | Argassi beach Zakynthos, Greece<br>6.94 g<br>26.4293 mm<br>0.690498<br>3 | 2885.04 mm <sup>3</sup><br>18.8354 mm<br>0.71267<br>2  | 1093.48 mm <sup>2</sup><br>13.0058 mm<br>sphere<br>3 | 0.719993                             | 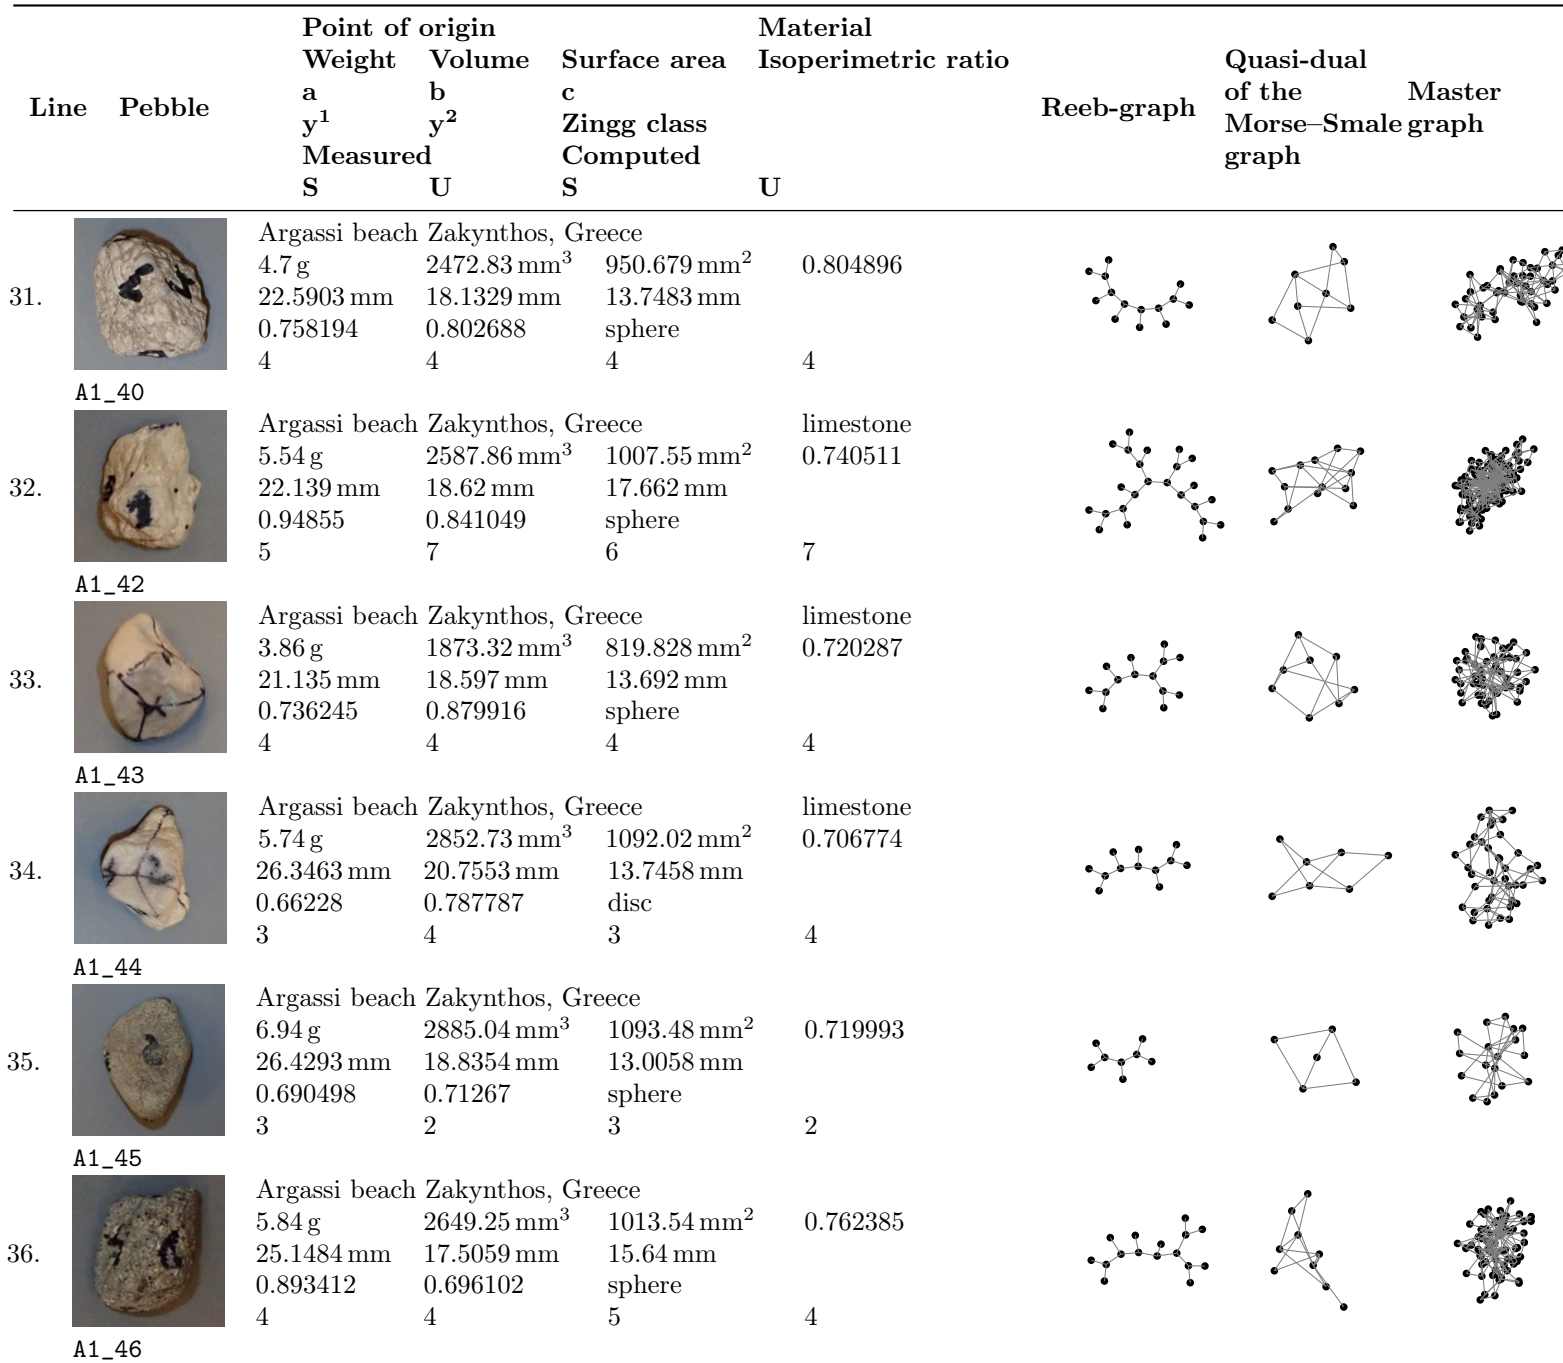 | 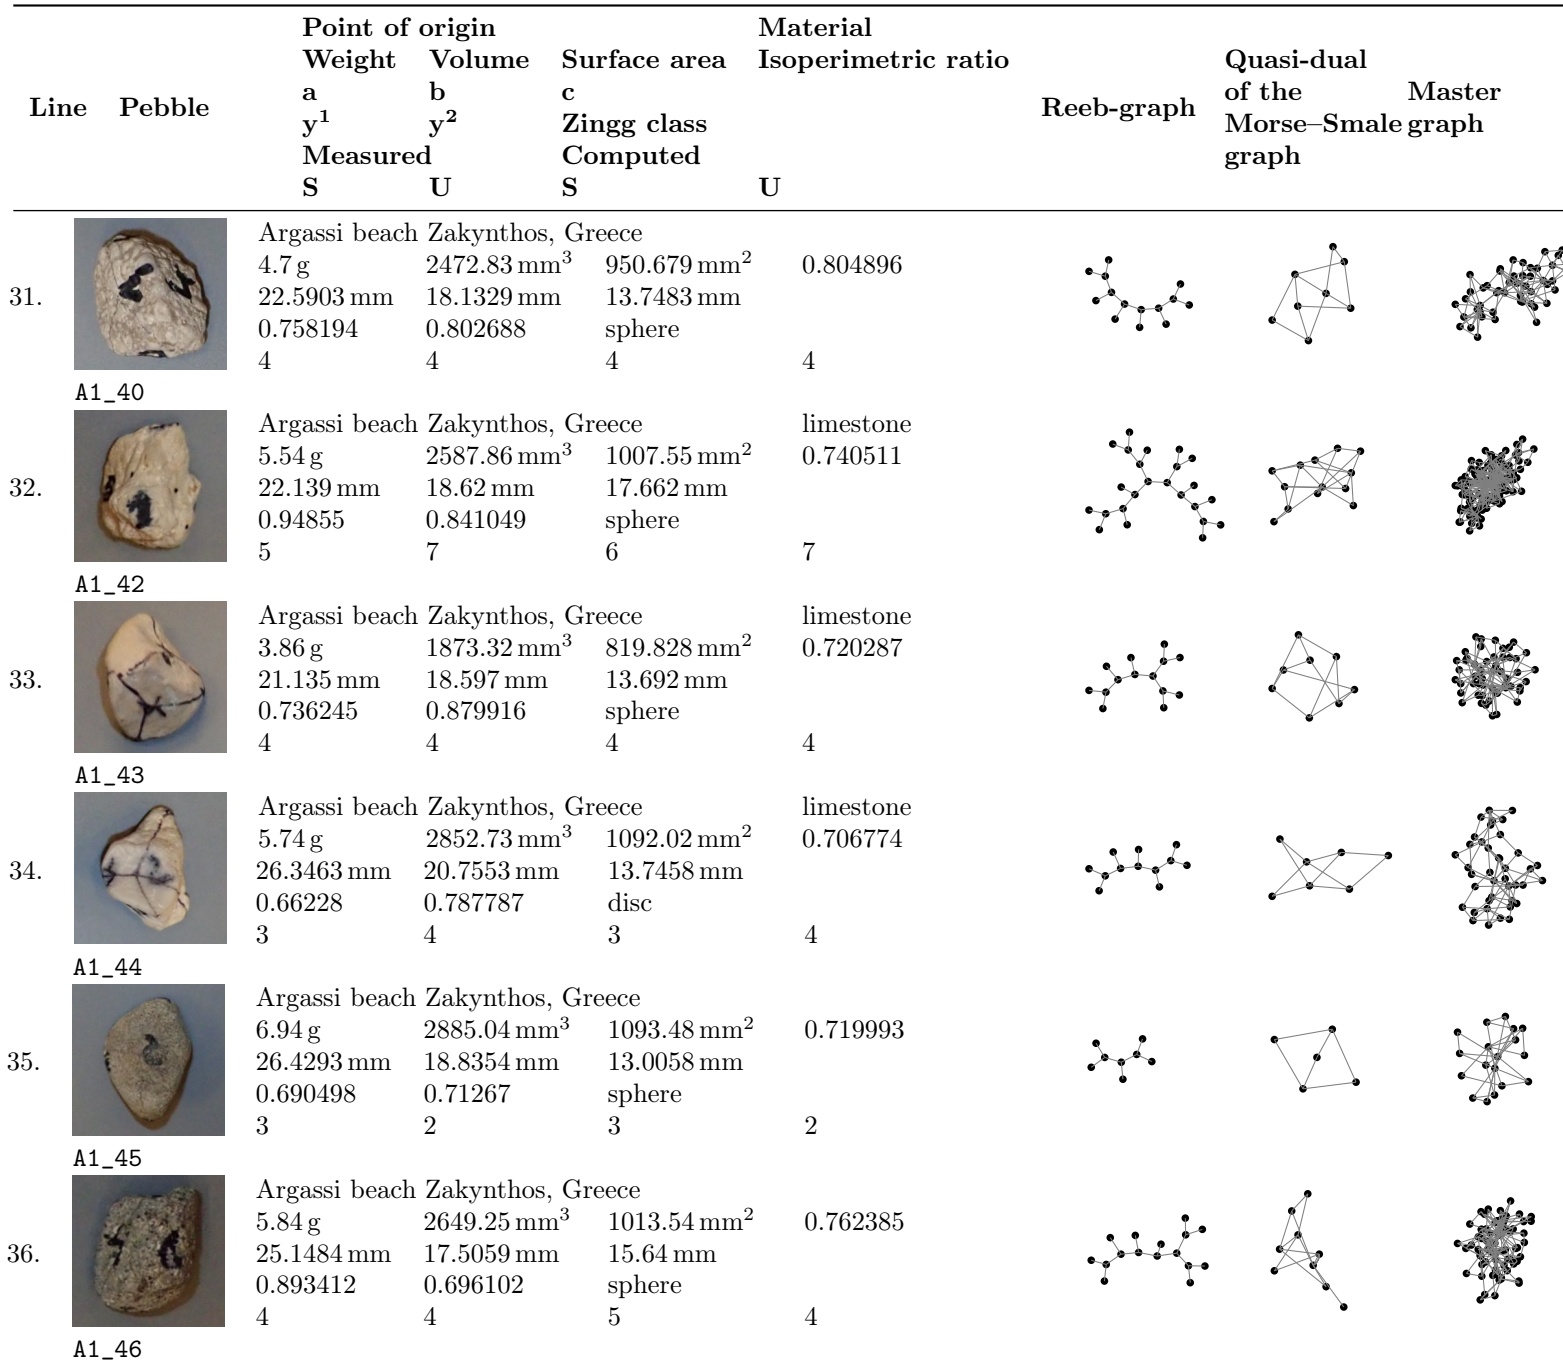 | 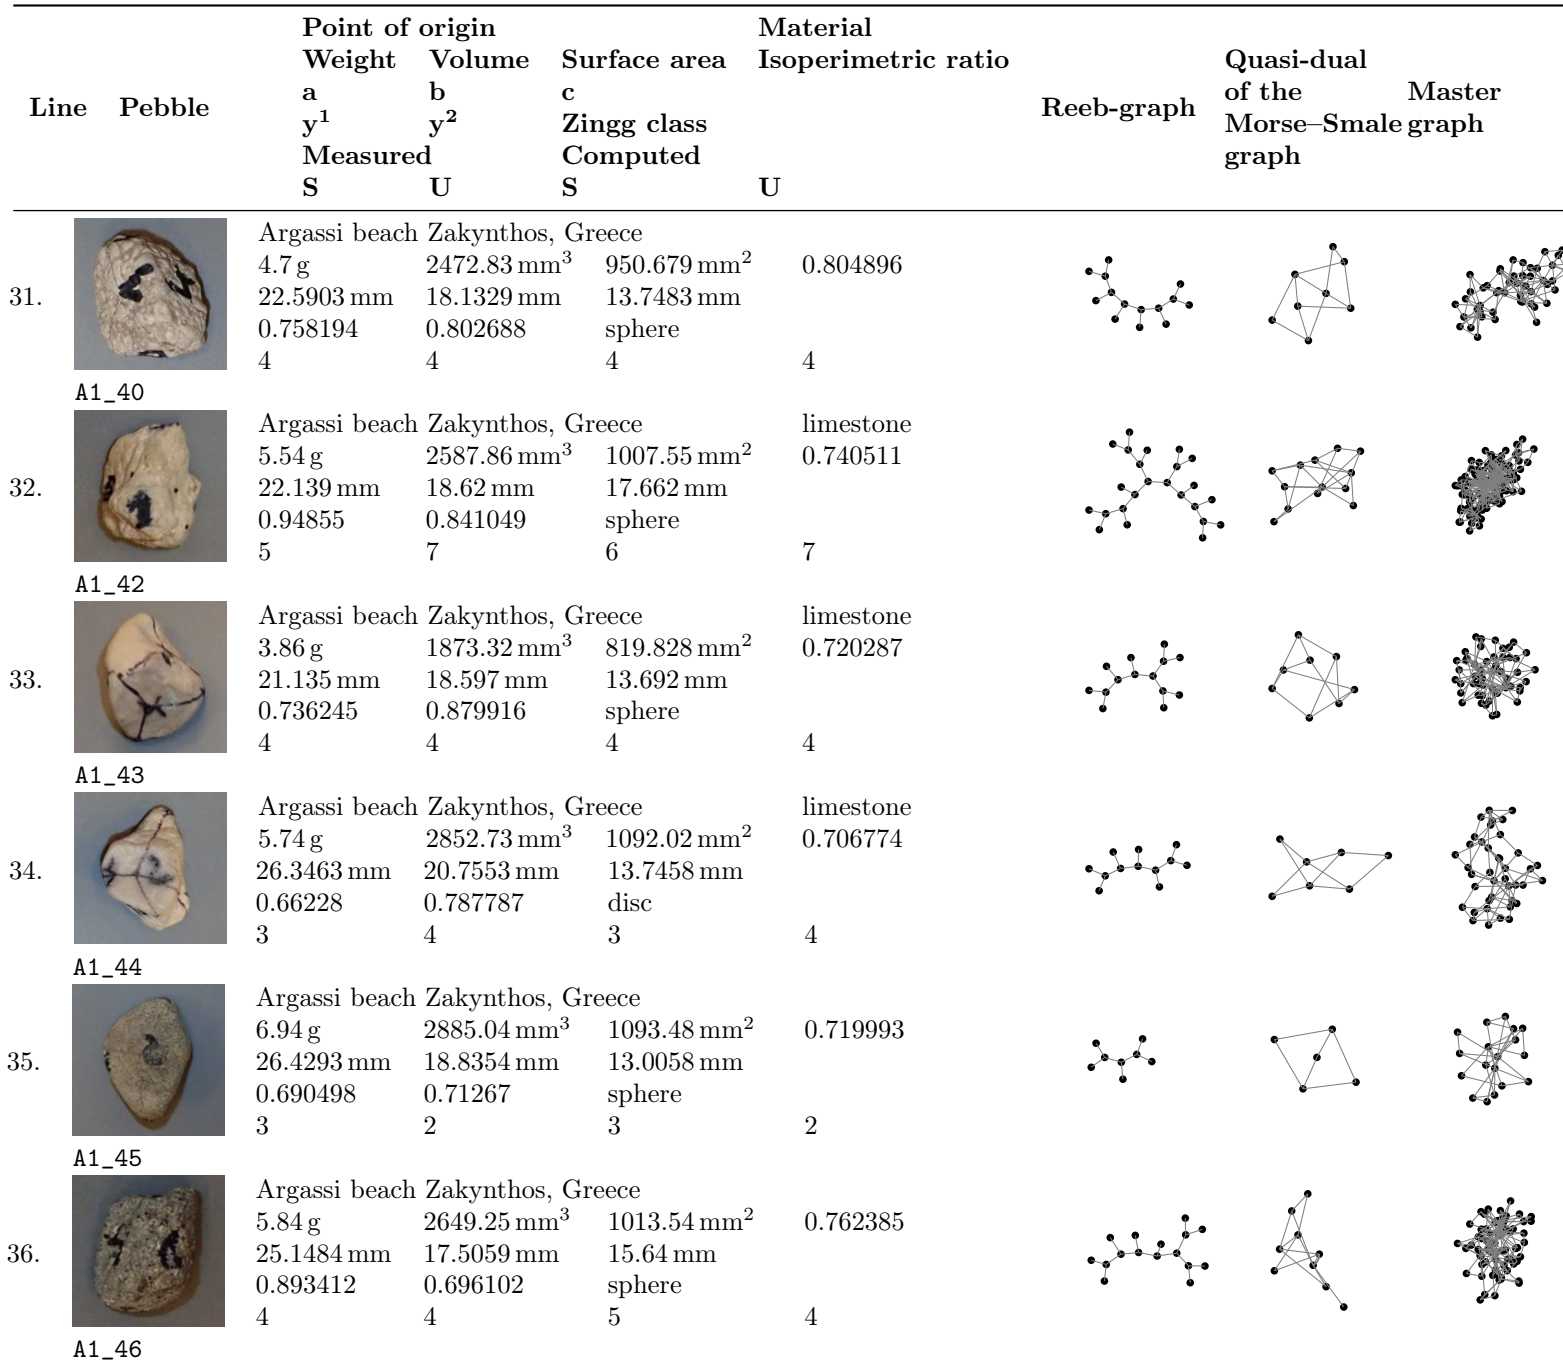 |
|      | A1_45                                                                               |                                                                          |                                                        |                                                      |                                      |                                                                                       |                                                                                       |                                                                                       |
| 36.  | 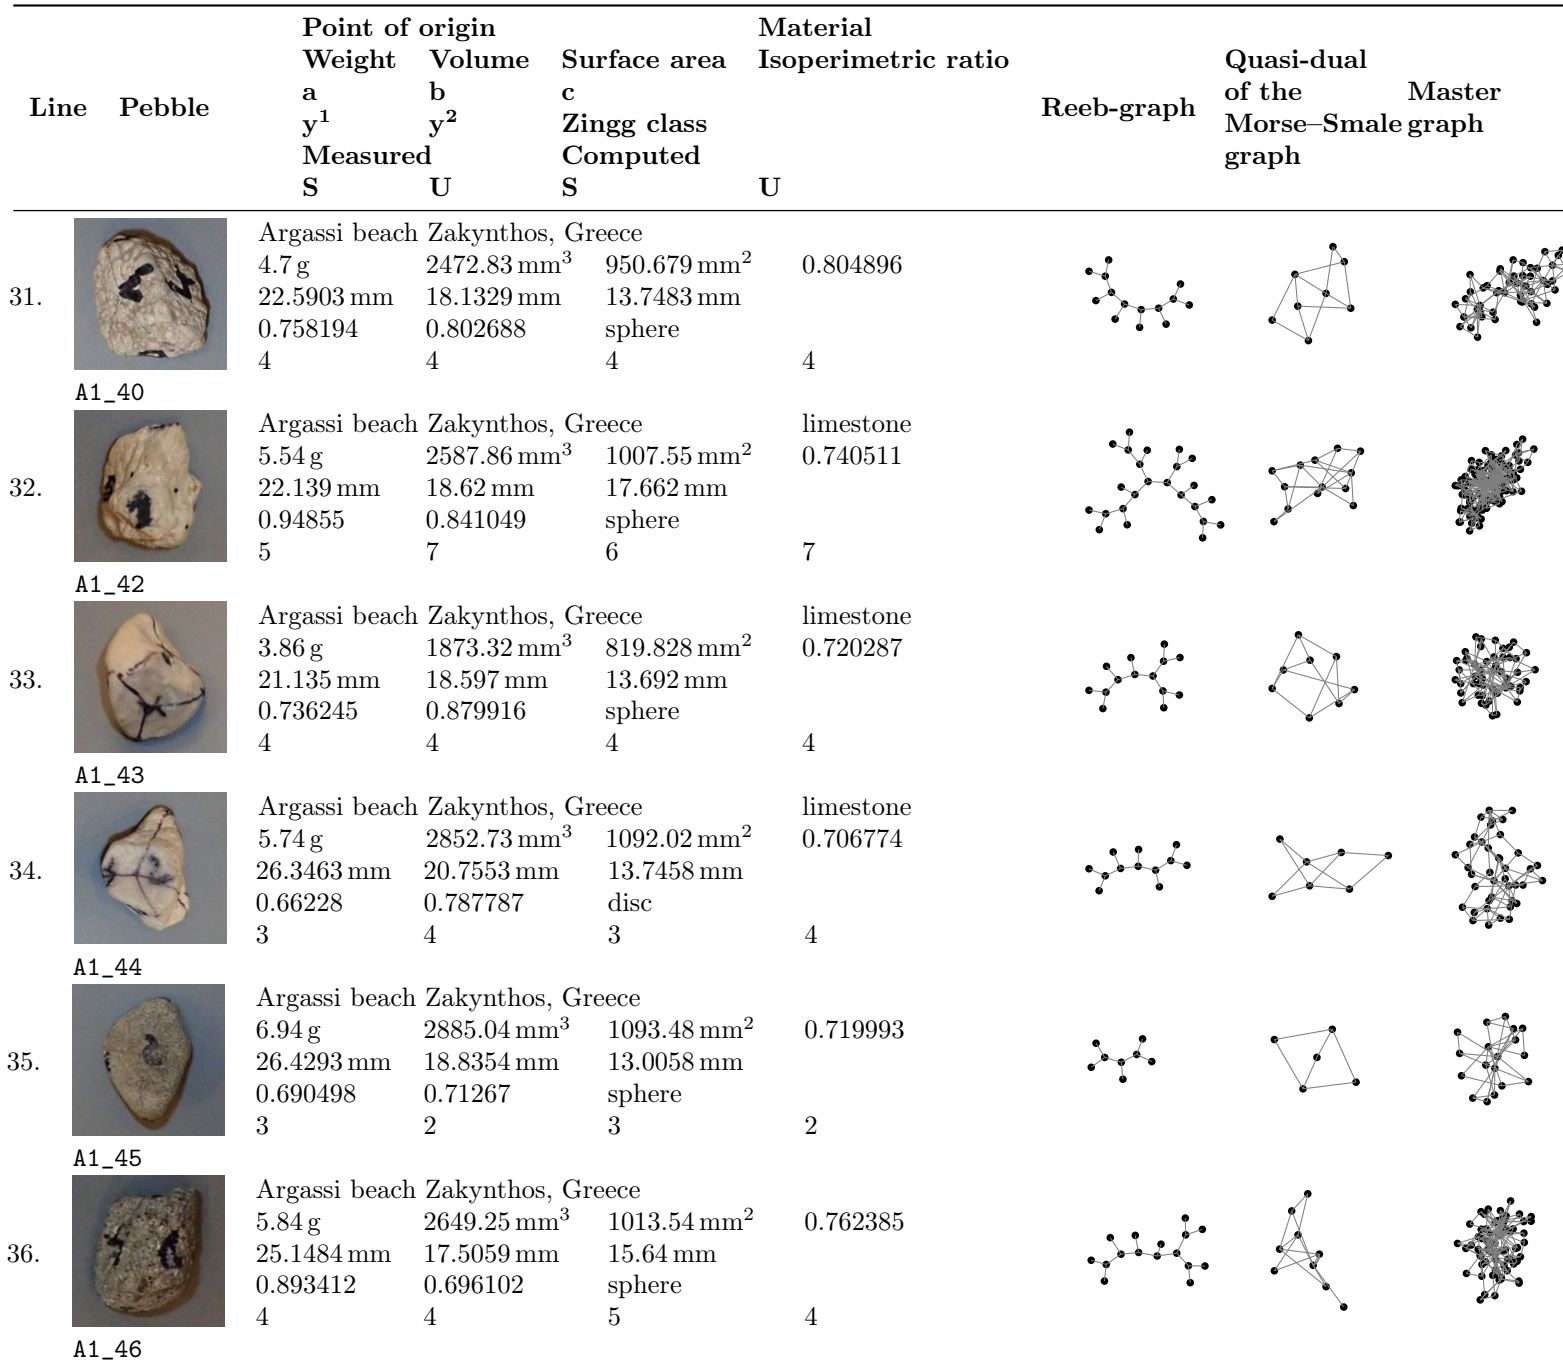 | Argassi beach Zakynthos, Greece<br>5.84 g<br>25.1484 mm<br>0.893412<br>4 | 2649.25 mm <sup>3</sup><br>17.5059 mm<br>0.696102<br>4 | 1013.54 mm <sup>2</sup><br>15.64 mm<br>sphere<br>5   | 0.762385                             | 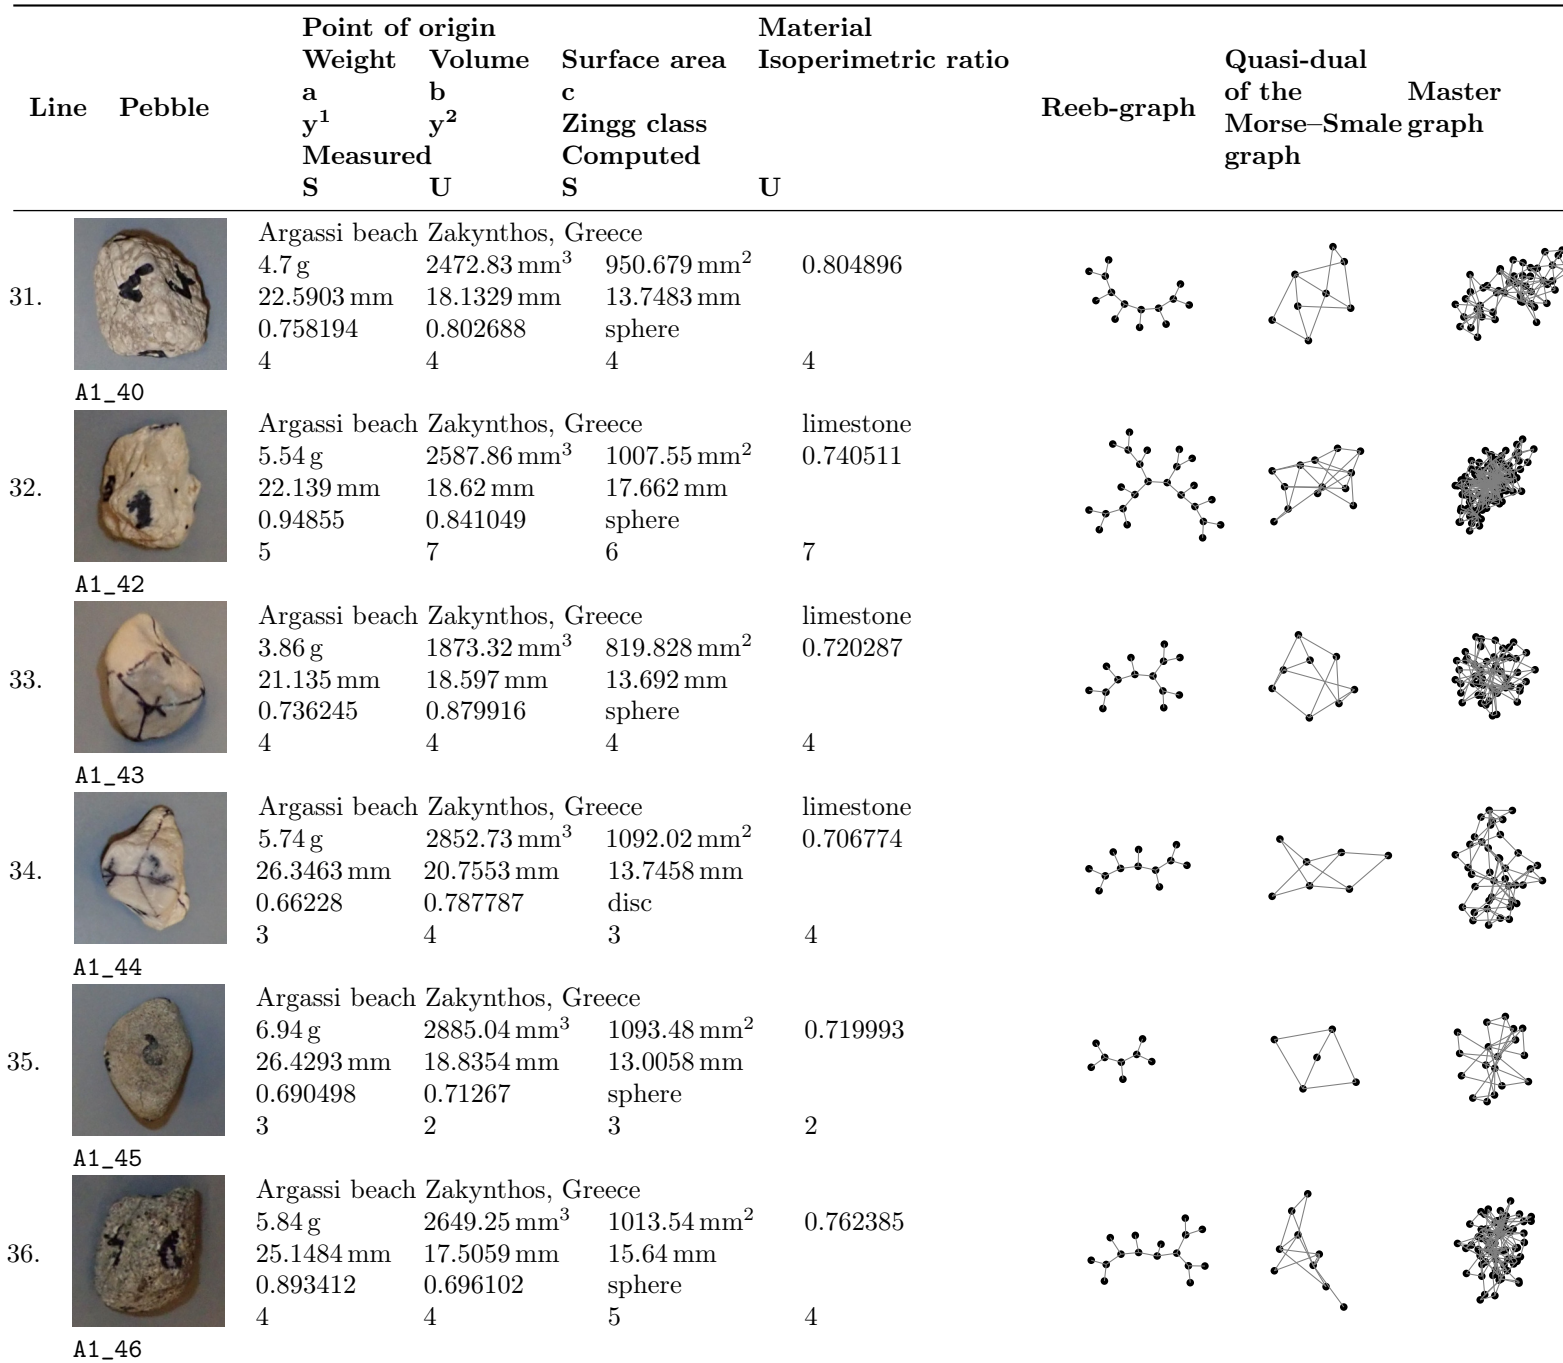 | 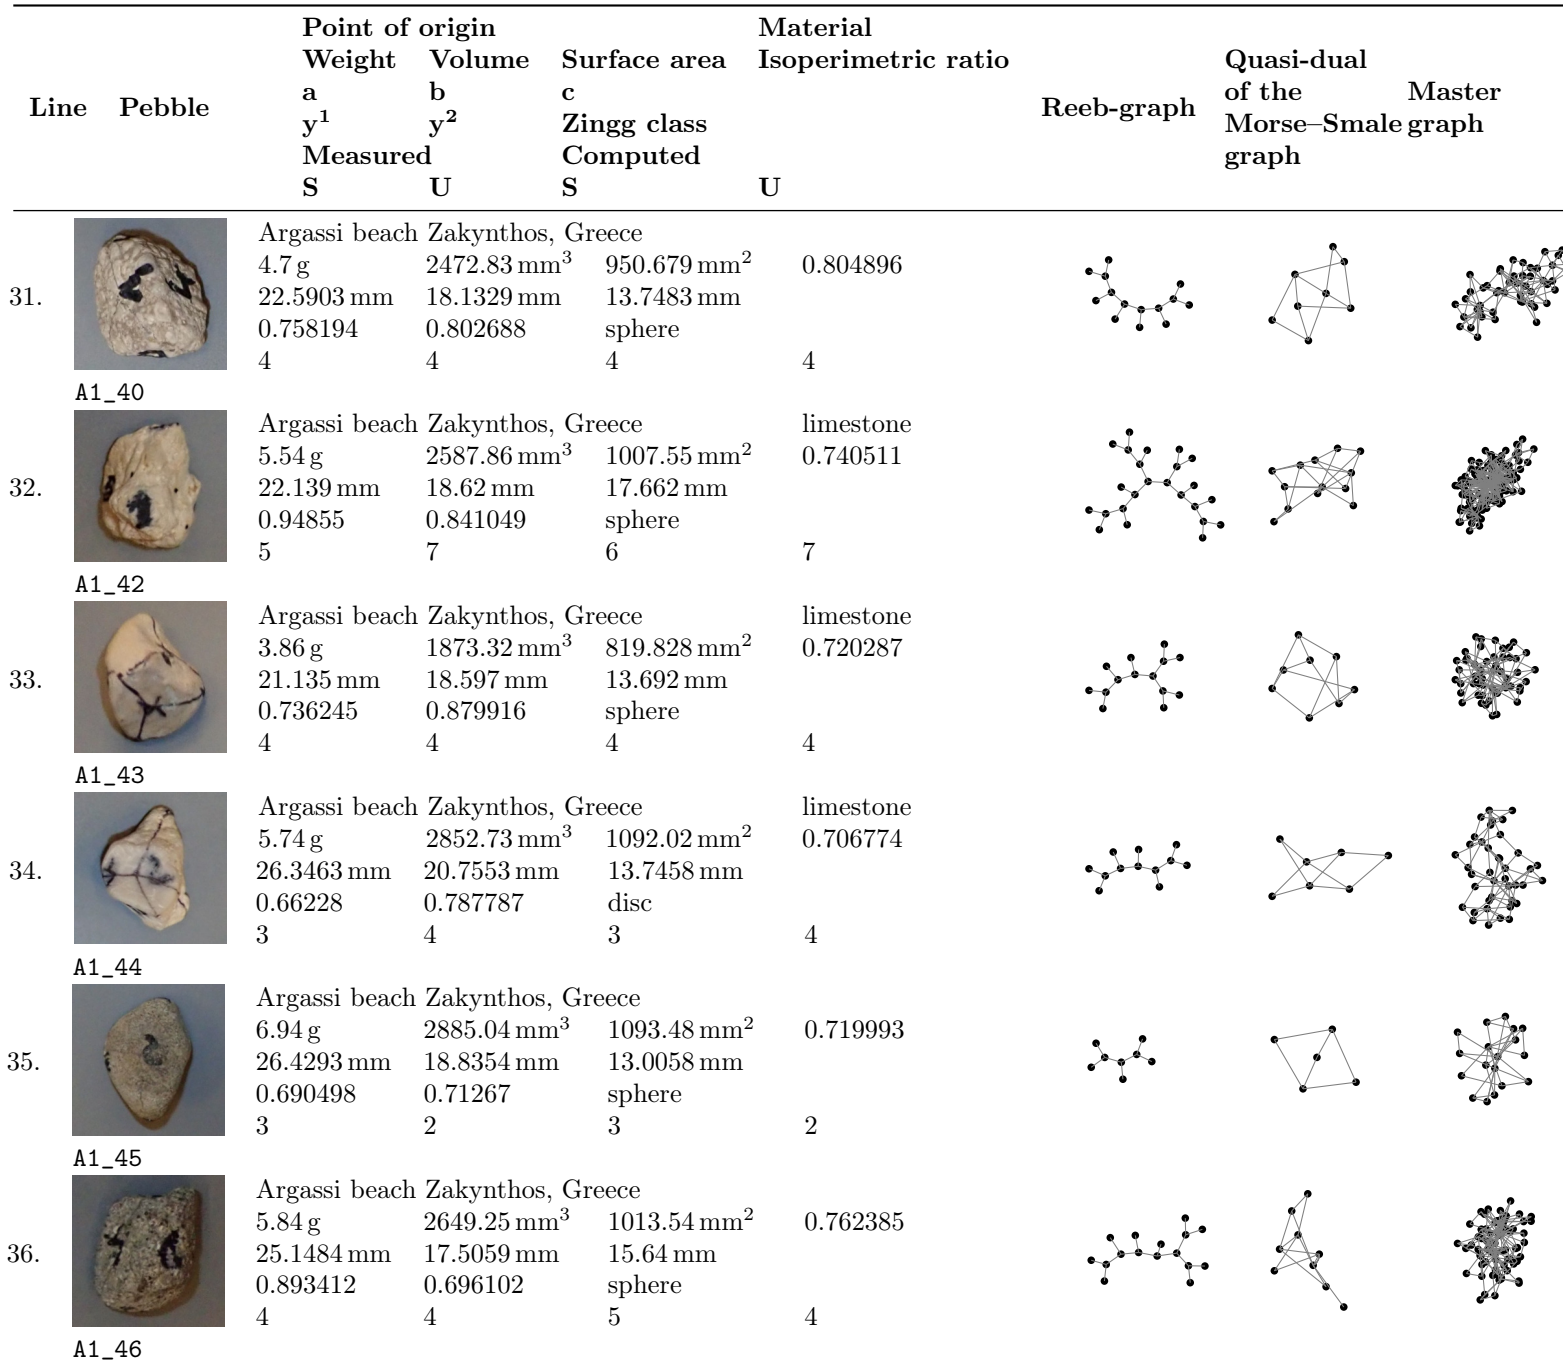 | 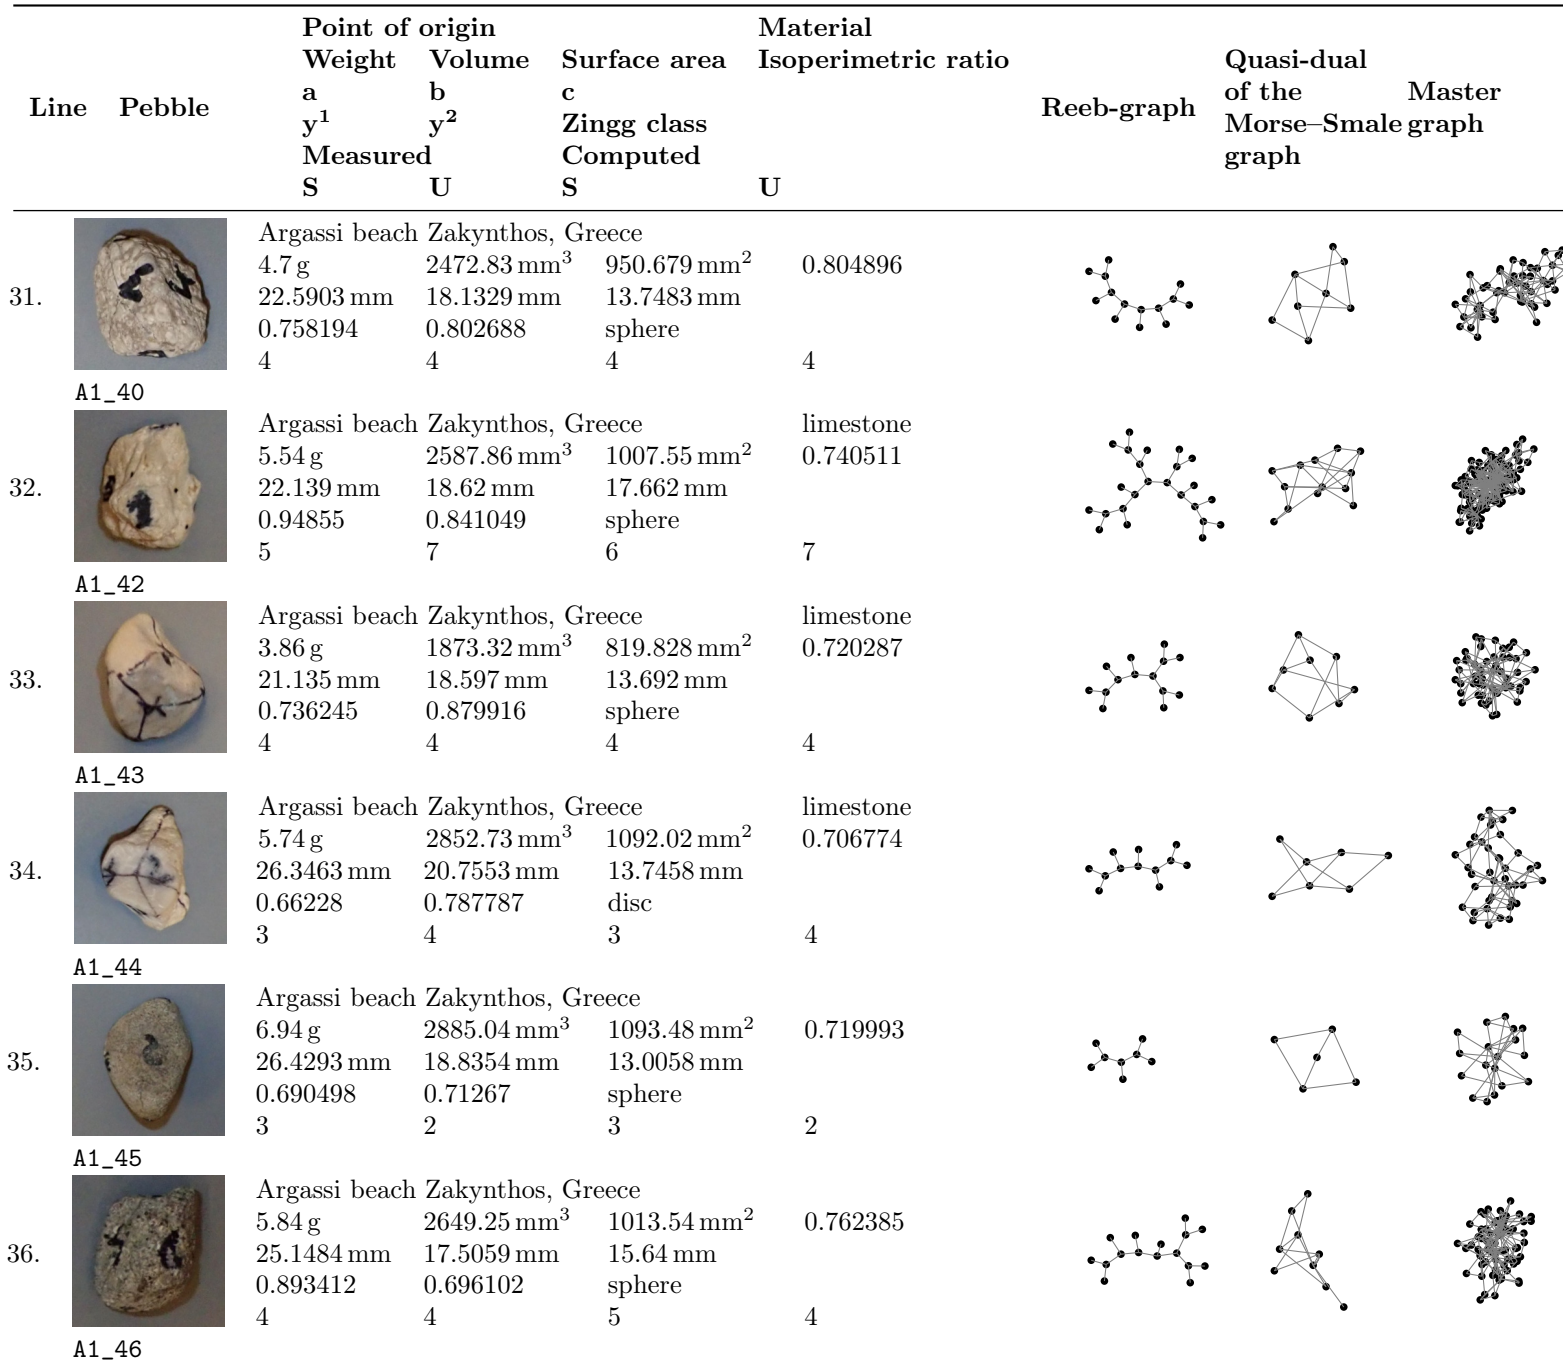 |
|      | A1_46                                                                               |                                                                          |                                                        |                                                      |                                      |                                                                                       |                                                                                       |                                                                                       |

| Line | Pebble                                                                              | Point of origin                      |                          | Surface area<br>c<br>Zingg class<br>Computed<br>S    | Material<br>Isoperimetric ratio<br>U | Reeb-graph                                                                            | Quasi-dual<br>of the<br>Morse–Smale<br>graph                                          | Master<br>graph                                                                       |
|------|-------------------------------------------------------------------------------------|--------------------------------------|--------------------------|------------------------------------------------------|--------------------------------------|---------------------------------------------------------------------------------------|---------------------------------------------------------------------------------------|---------------------------------------------------------------------------------------|
|      |                                                                                     | Weight                               | Volume                   |                                                      |                                      |                                                                                       |                                                                                       |                                                                                       |
|      |                                                                                     | a<br>y <sup>1</sup><br>Measured<br>S | b<br>y <sup>2</sup><br>U |                                                      |                                      |                                                                                       |                                                                                       |                                                                                       |
|      |                                                                                     |                                      |                          |                                                      |                                      |                                                                                       |                                                                                       |                                                                                       |
| 37.  | 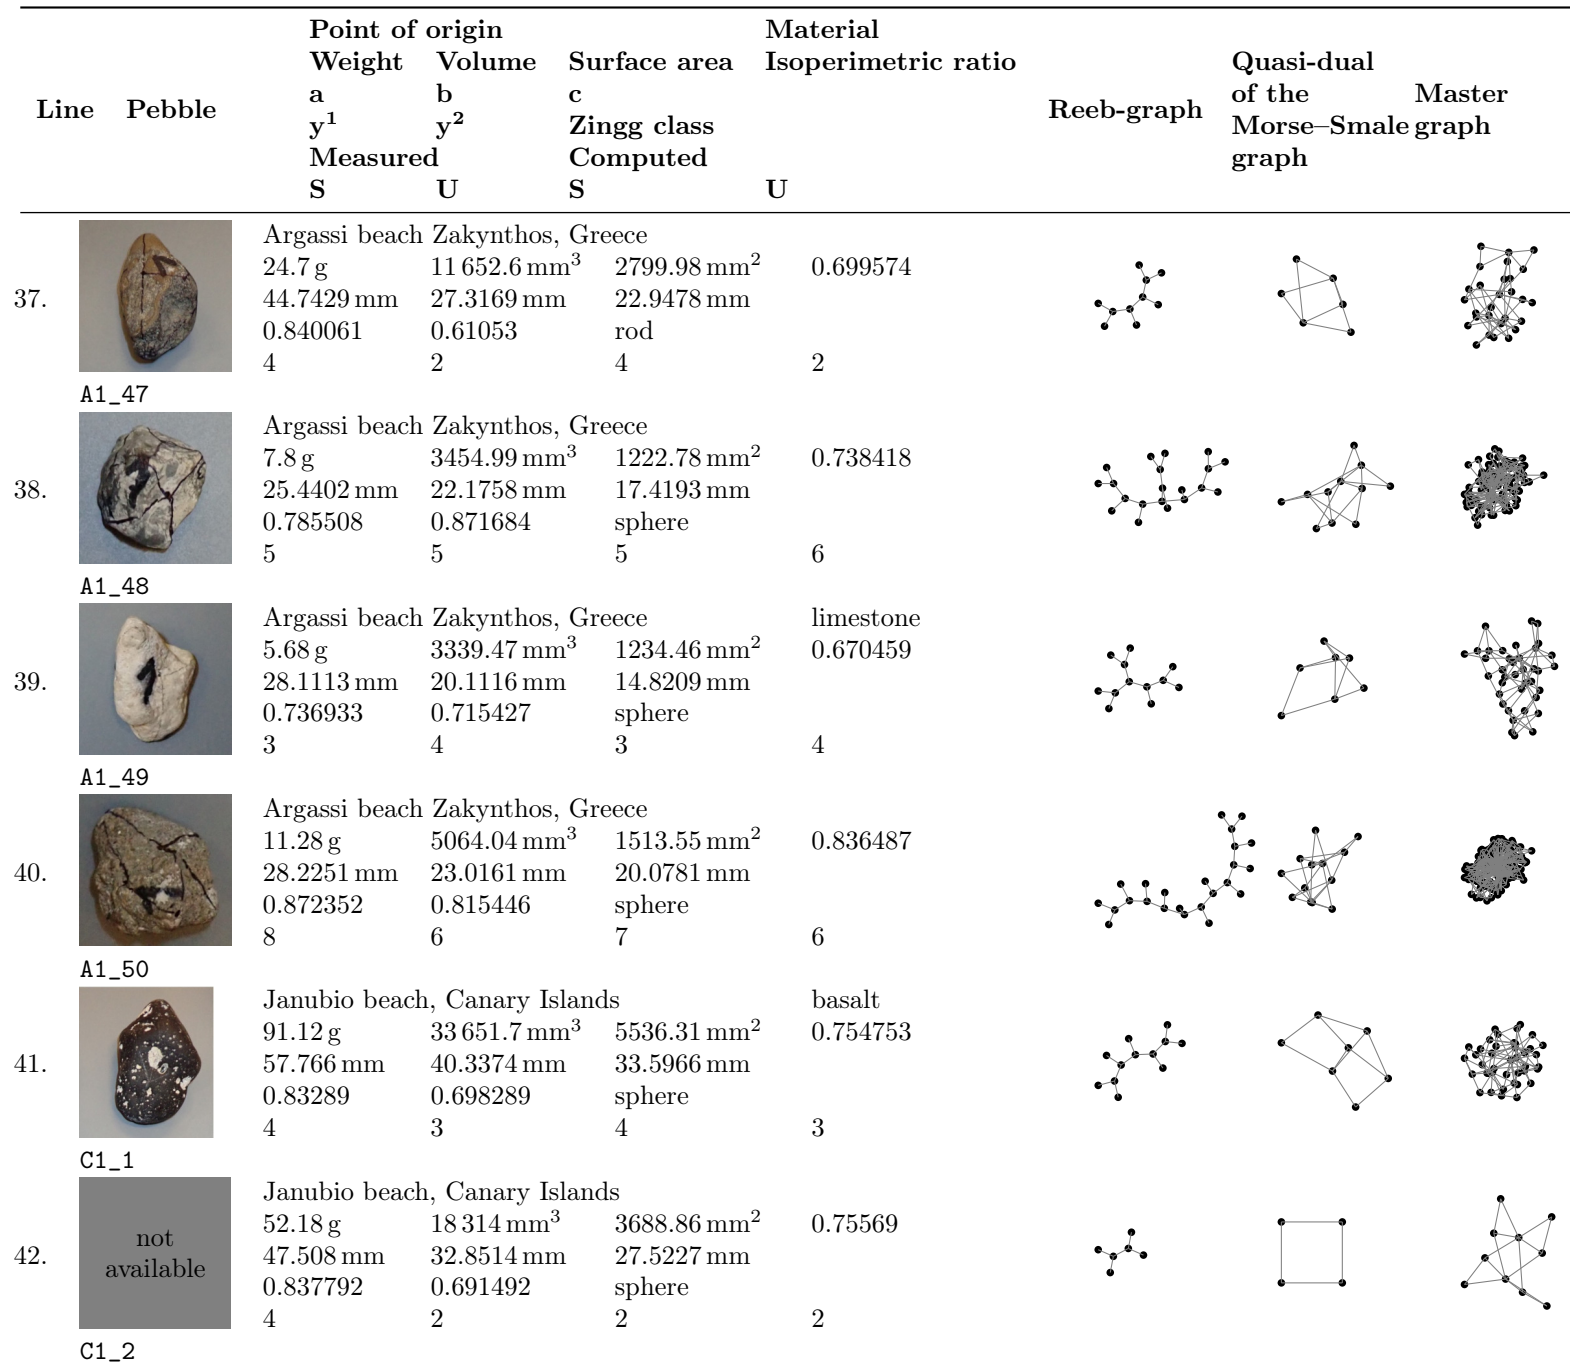   | Argassi beach Zakynthos, Greece      |                          | 2799.98 mm <sup>2</sup><br>22.9478 mm<br>rod<br>4    | 0.699574<br>2                        | 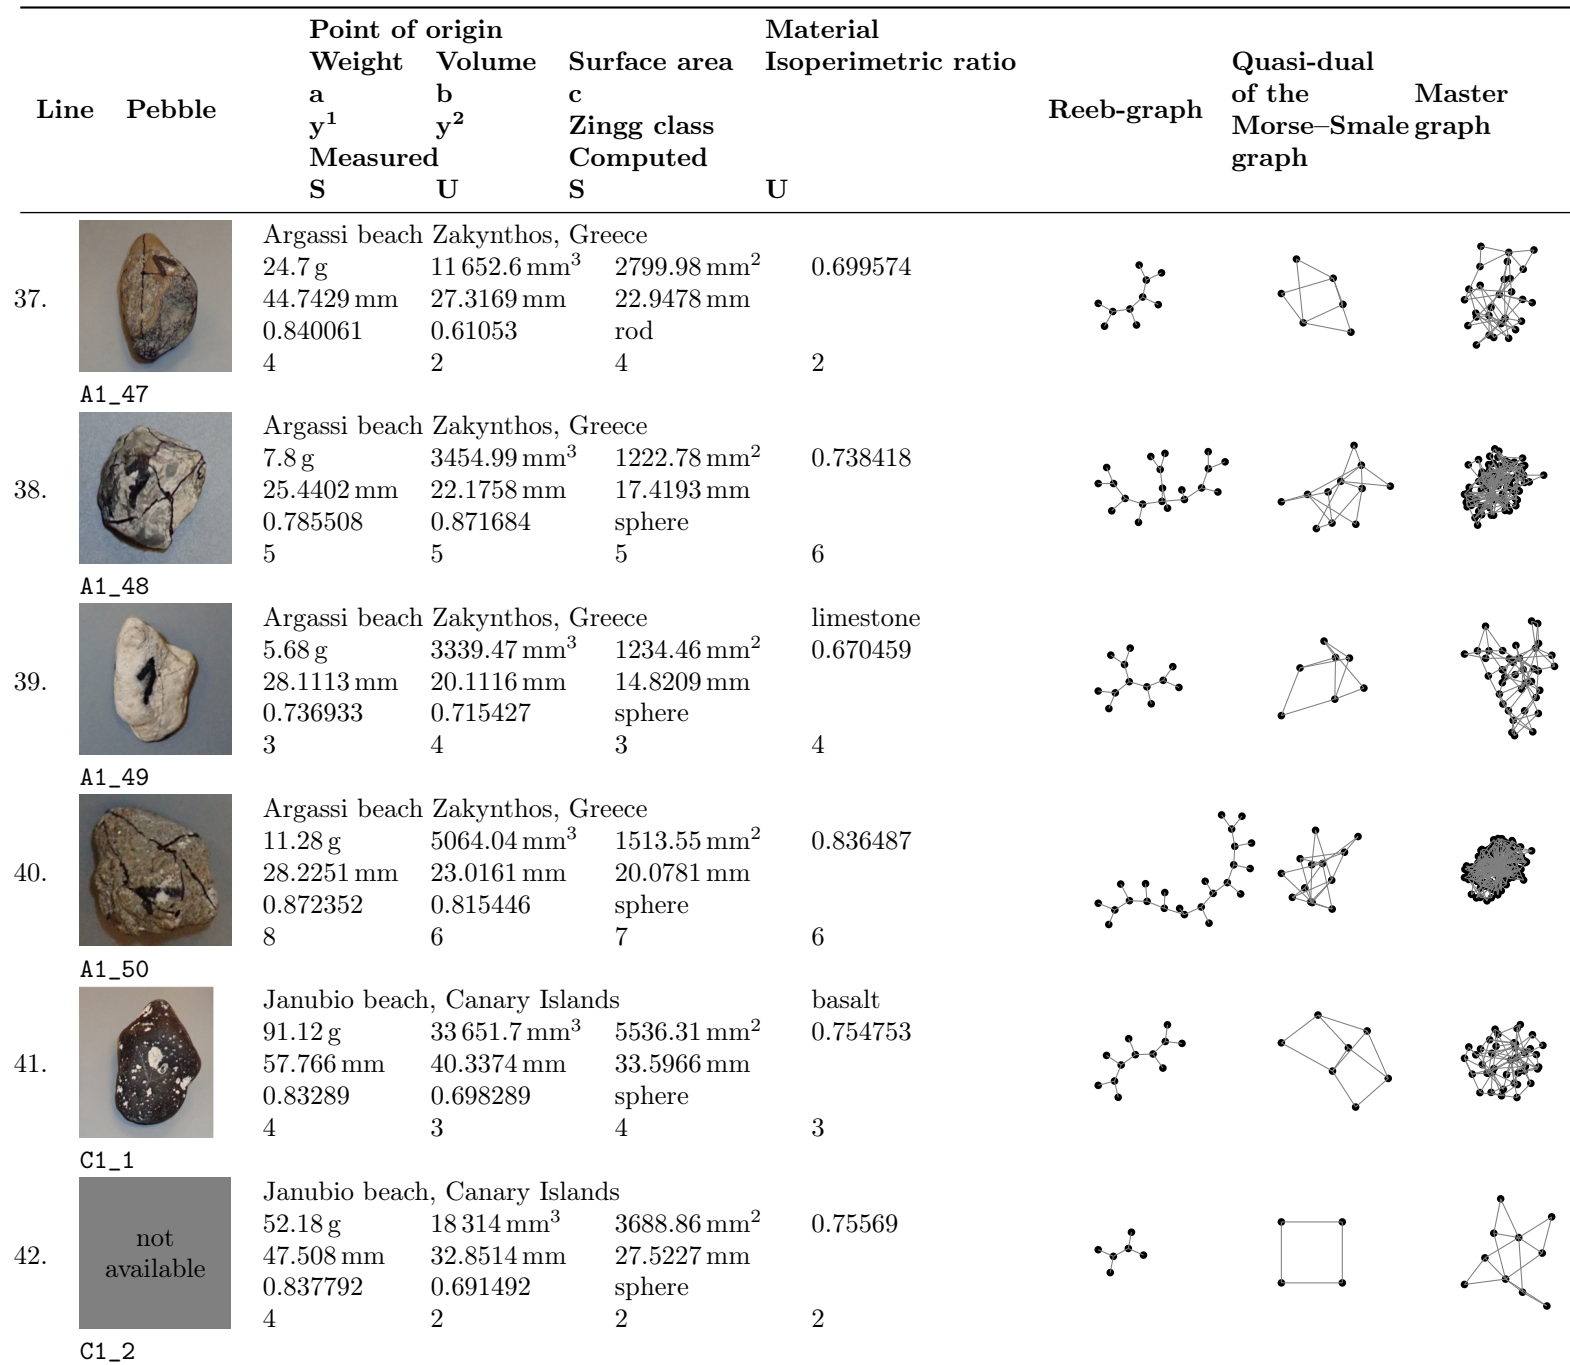   | 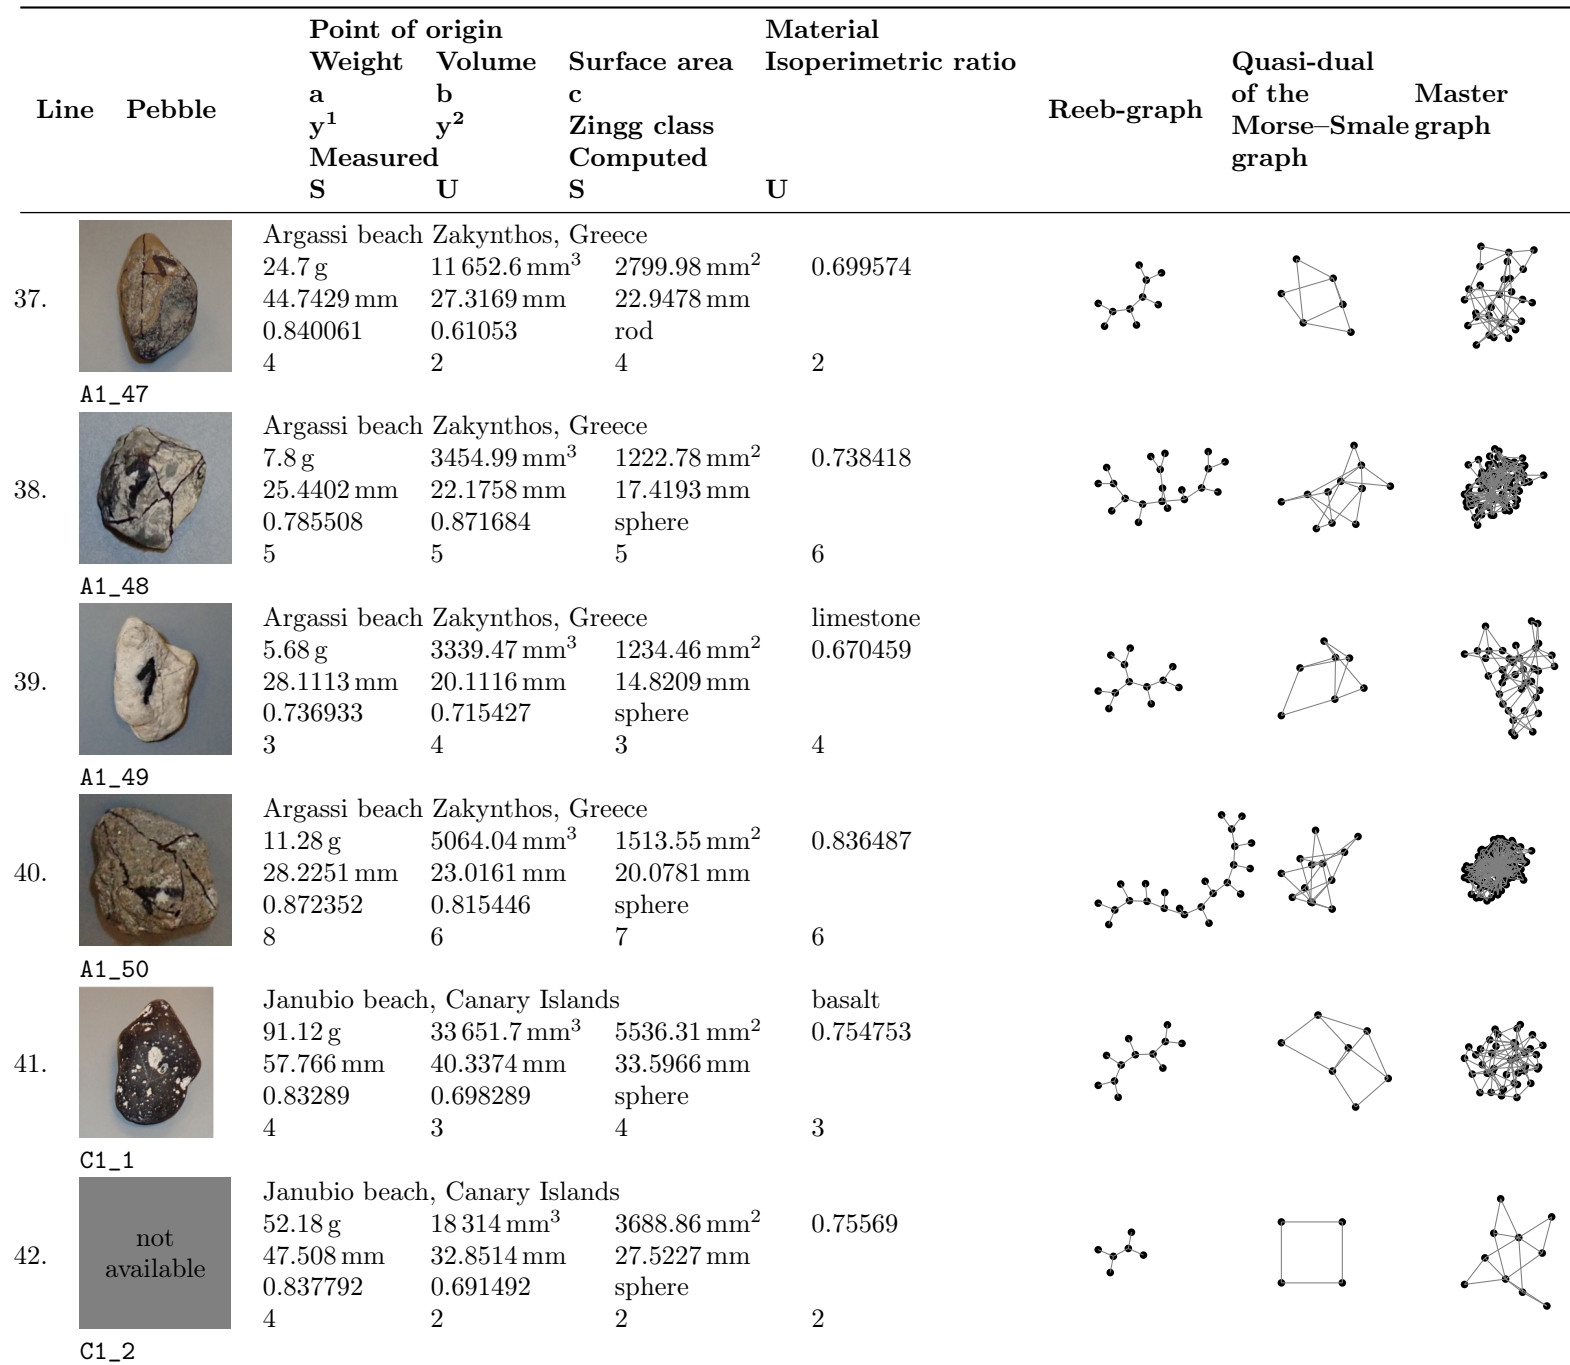   | 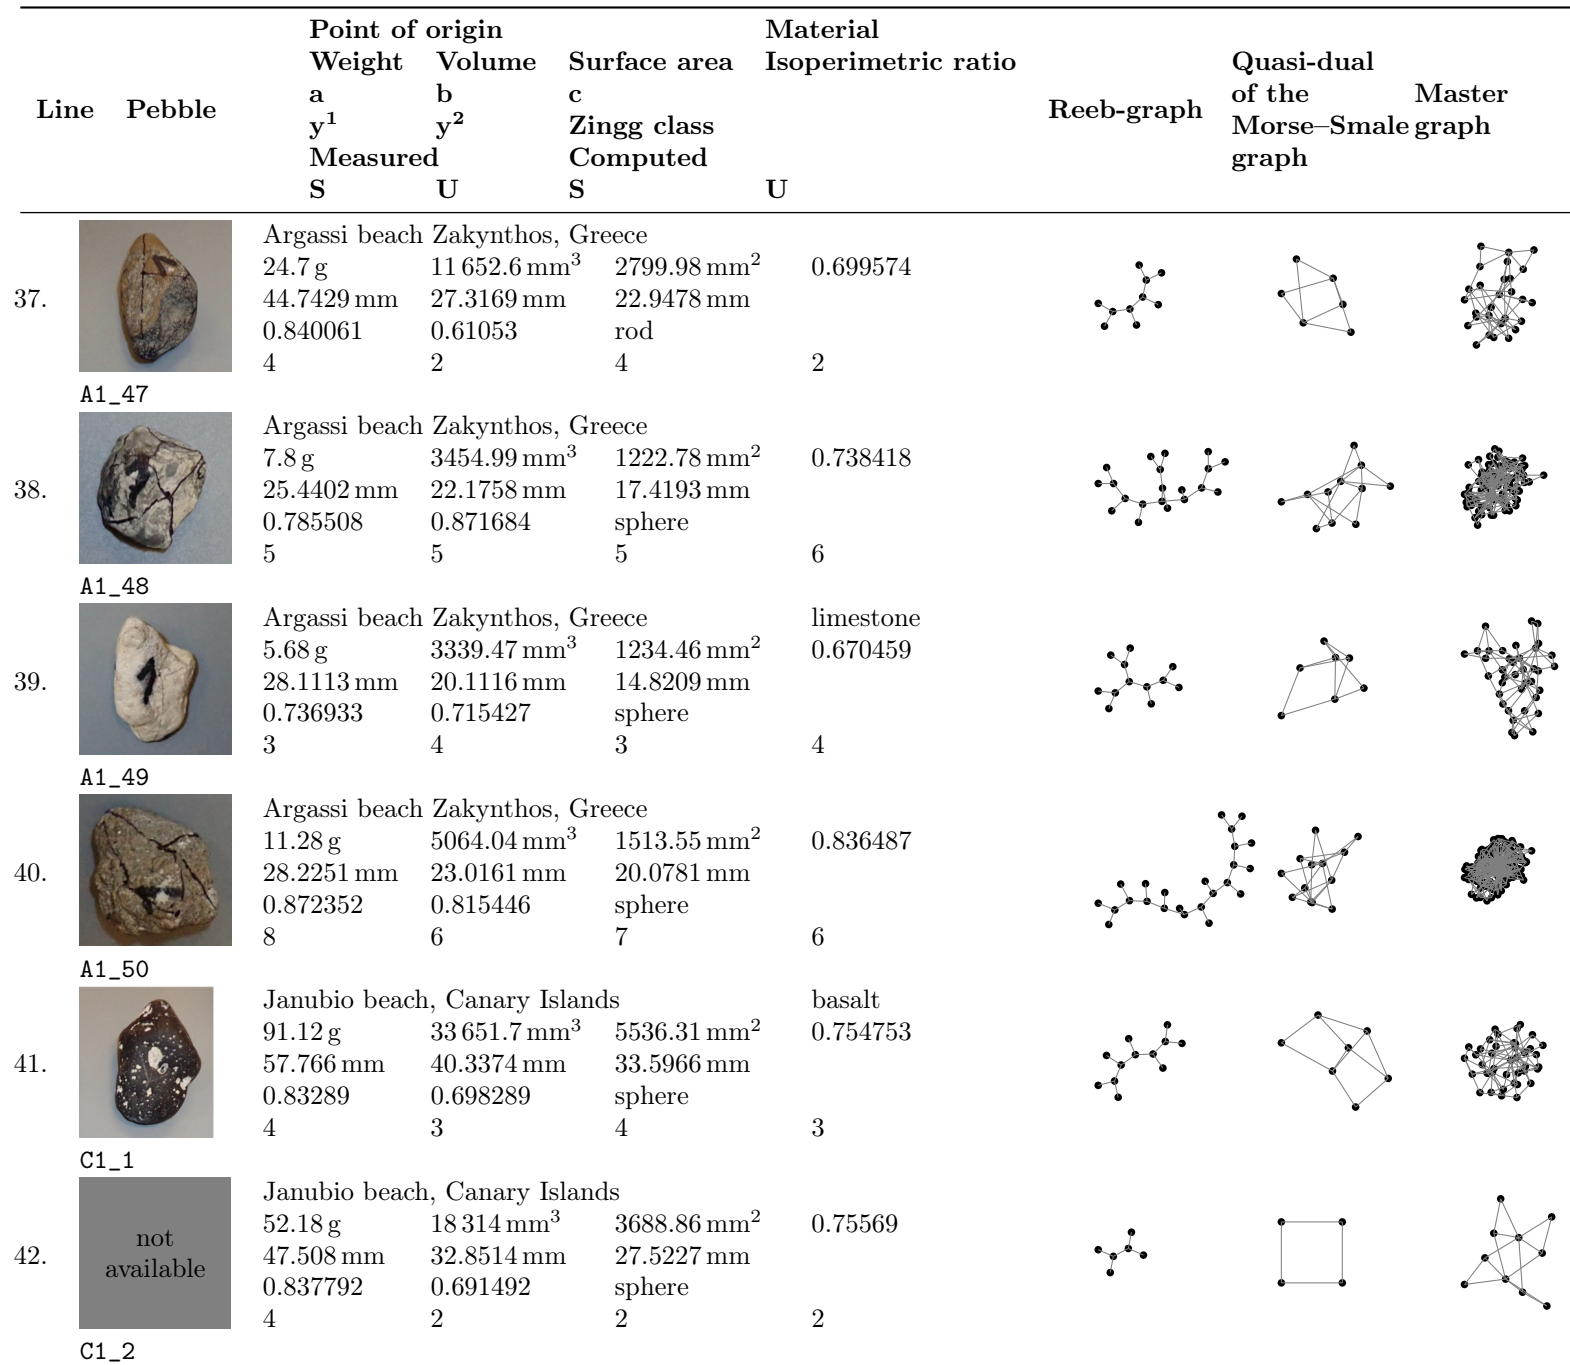   |
|      |                                                                                     | 24.7 g                               | 11 652.6 mm <sup>3</sup> |                                                      |                                      |                                                                                       |                                                                                       |                                                                                       |
|      |                                                                                     | 44.7429 mm                           | 27.3169 mm               |                                                      |                                      |                                                                                       |                                                                                       |                                                                                       |
|      |                                                                                     | 0.840061                             | 0.61053                  |                                                      |                                      |                                                                                       |                                                                                       |                                                                                       |
|      | A1_47                                                                               | 4                                    | 2                        |                                                      |                                      |                                                                                       |                                                                                       |                                                                                       |
| 38.  | 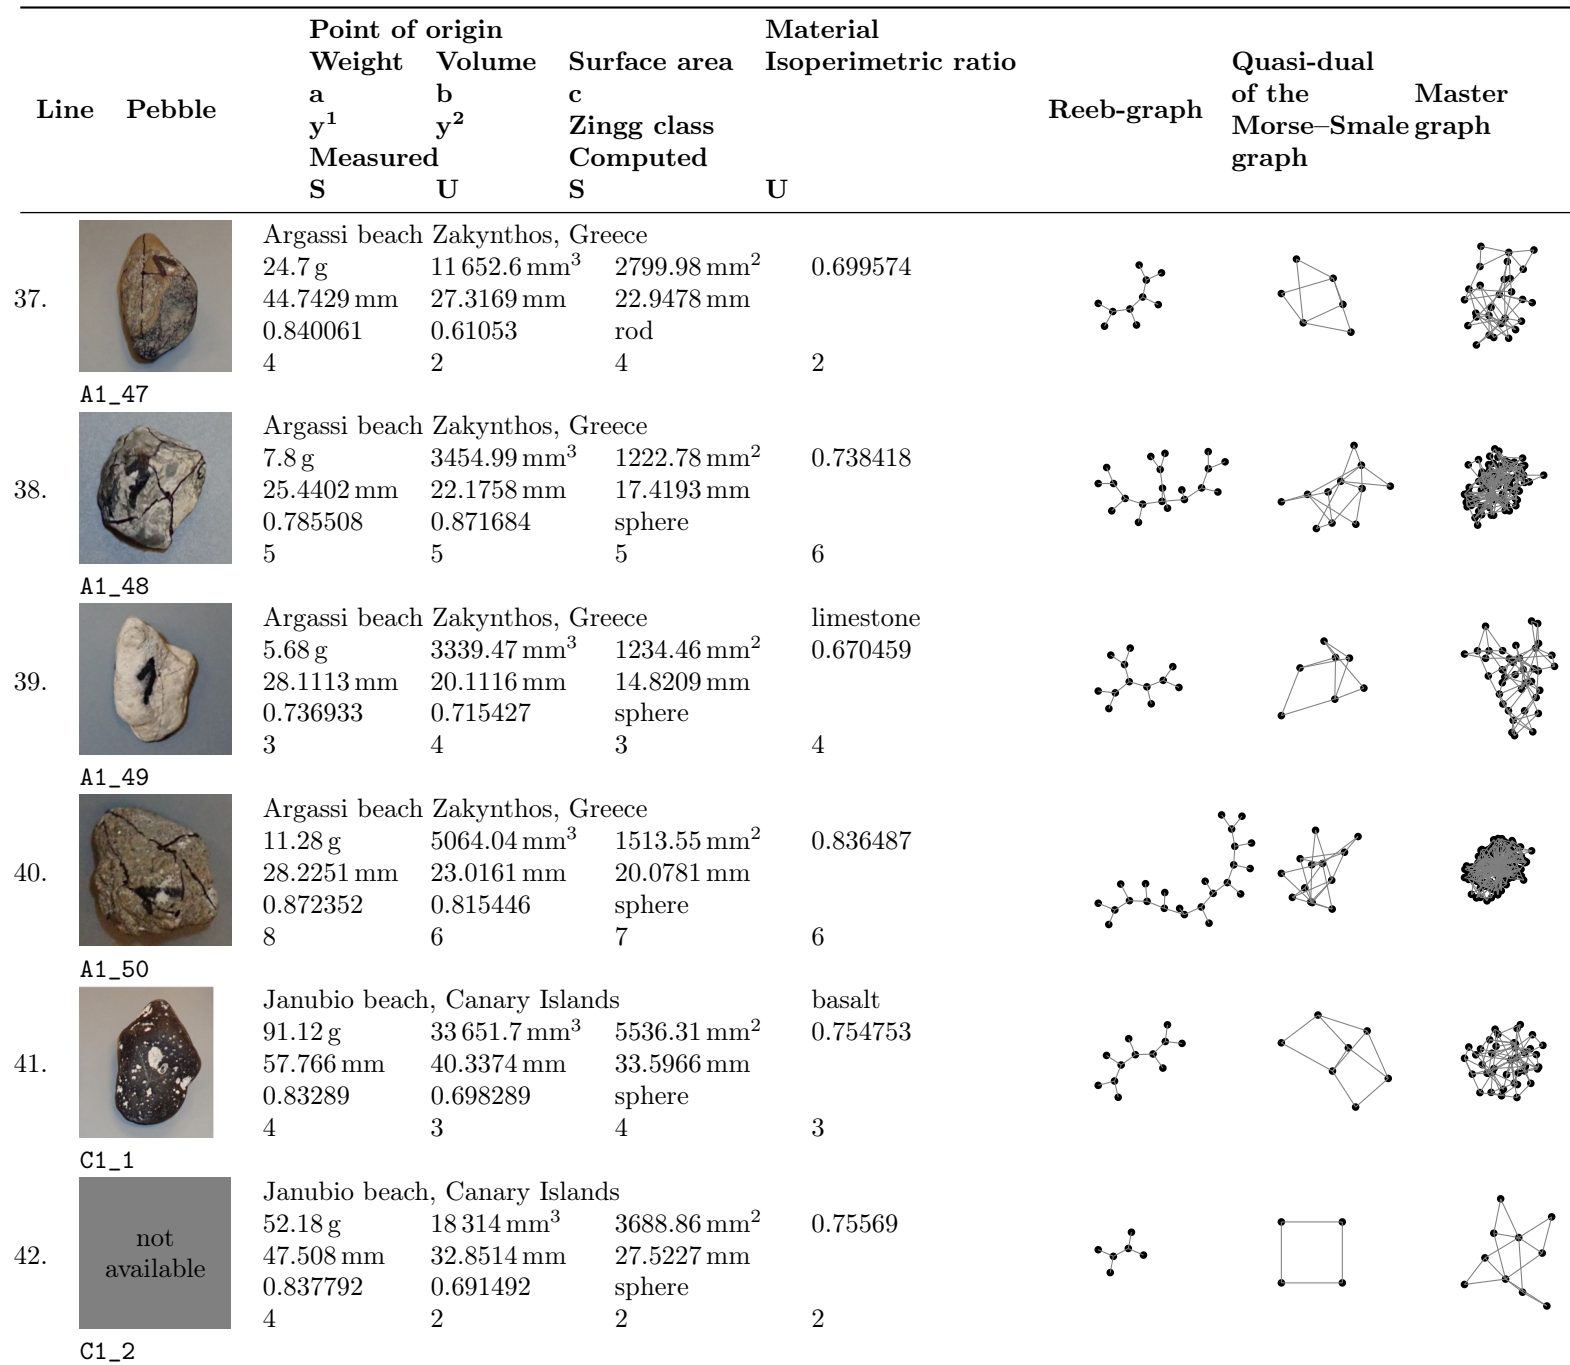   | Argassi beach Zakynthos, Greece      |                          | 1222.78 mm <sup>2</sup><br>17.4193 mm<br>sphere<br>5 | 0.738418<br>6                        | 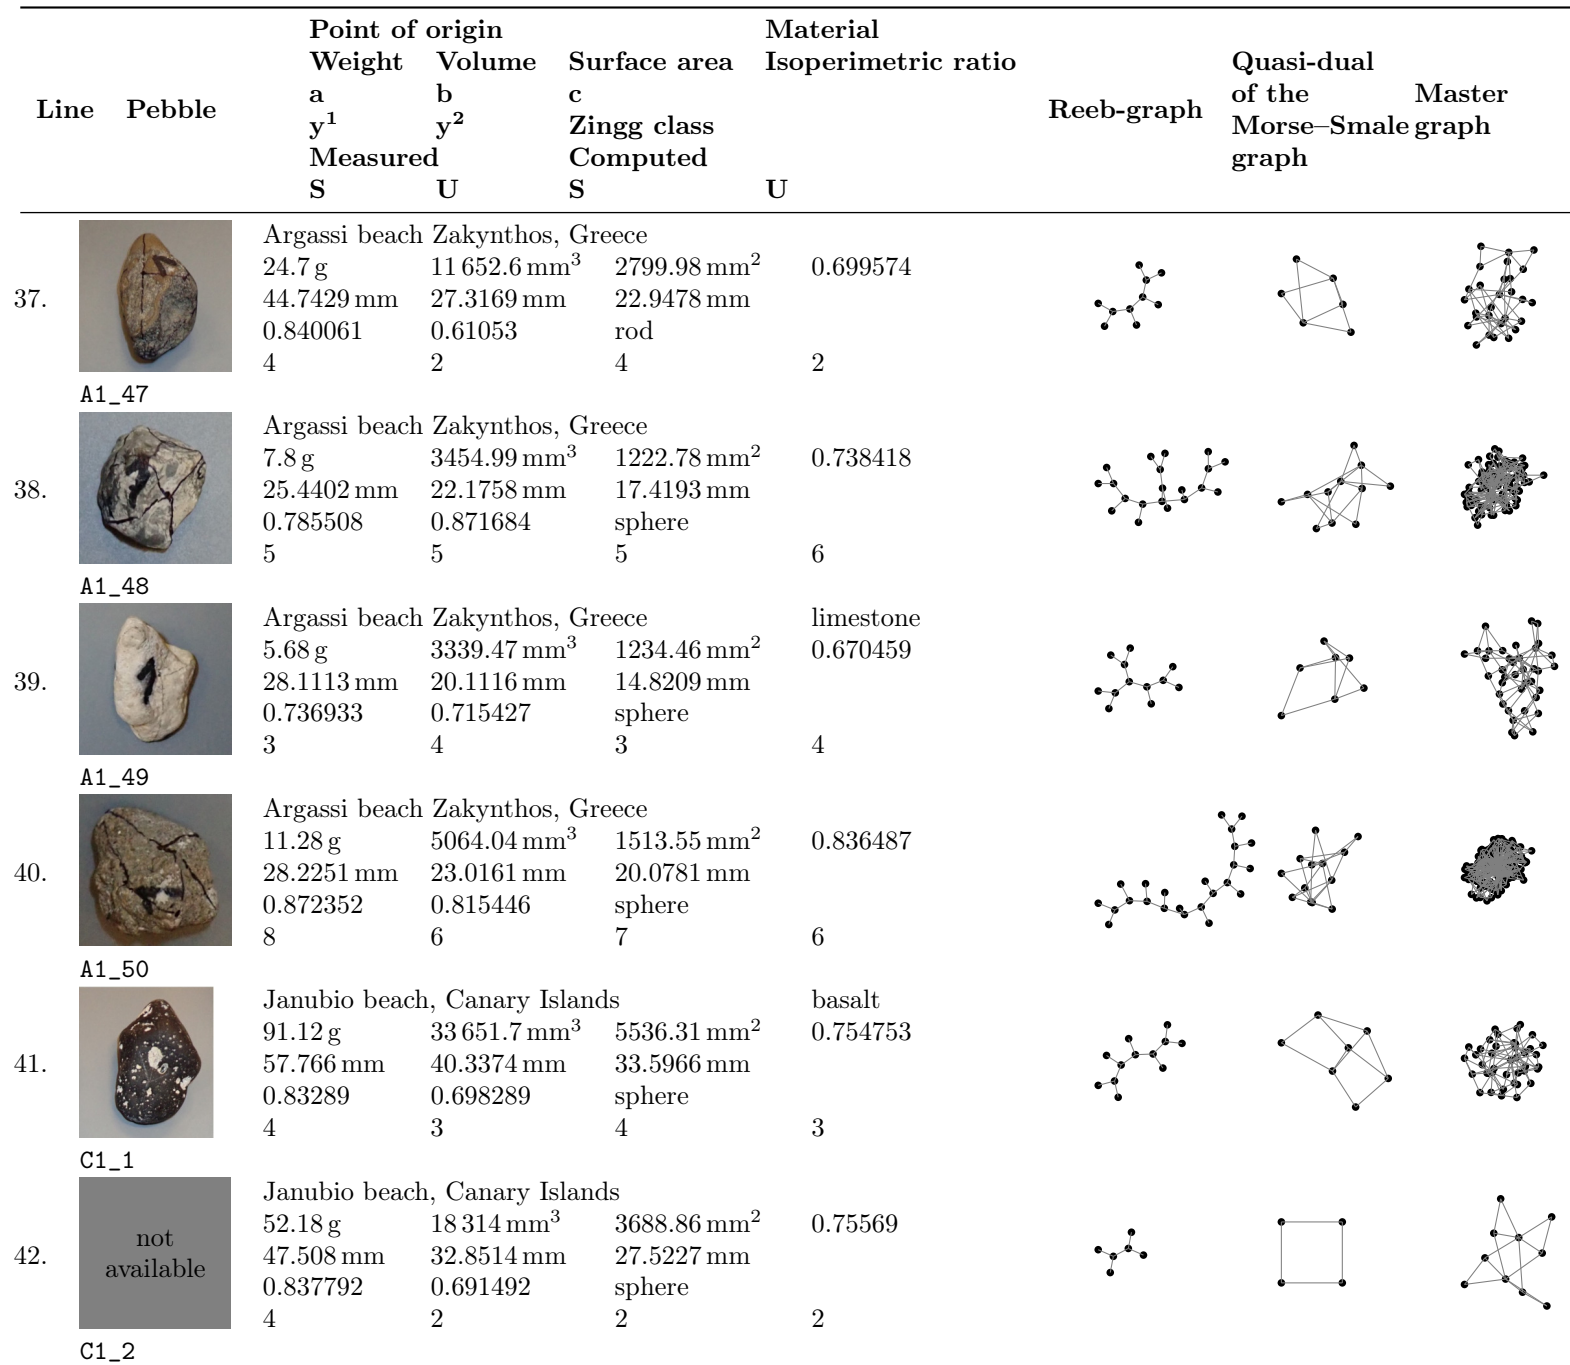   | 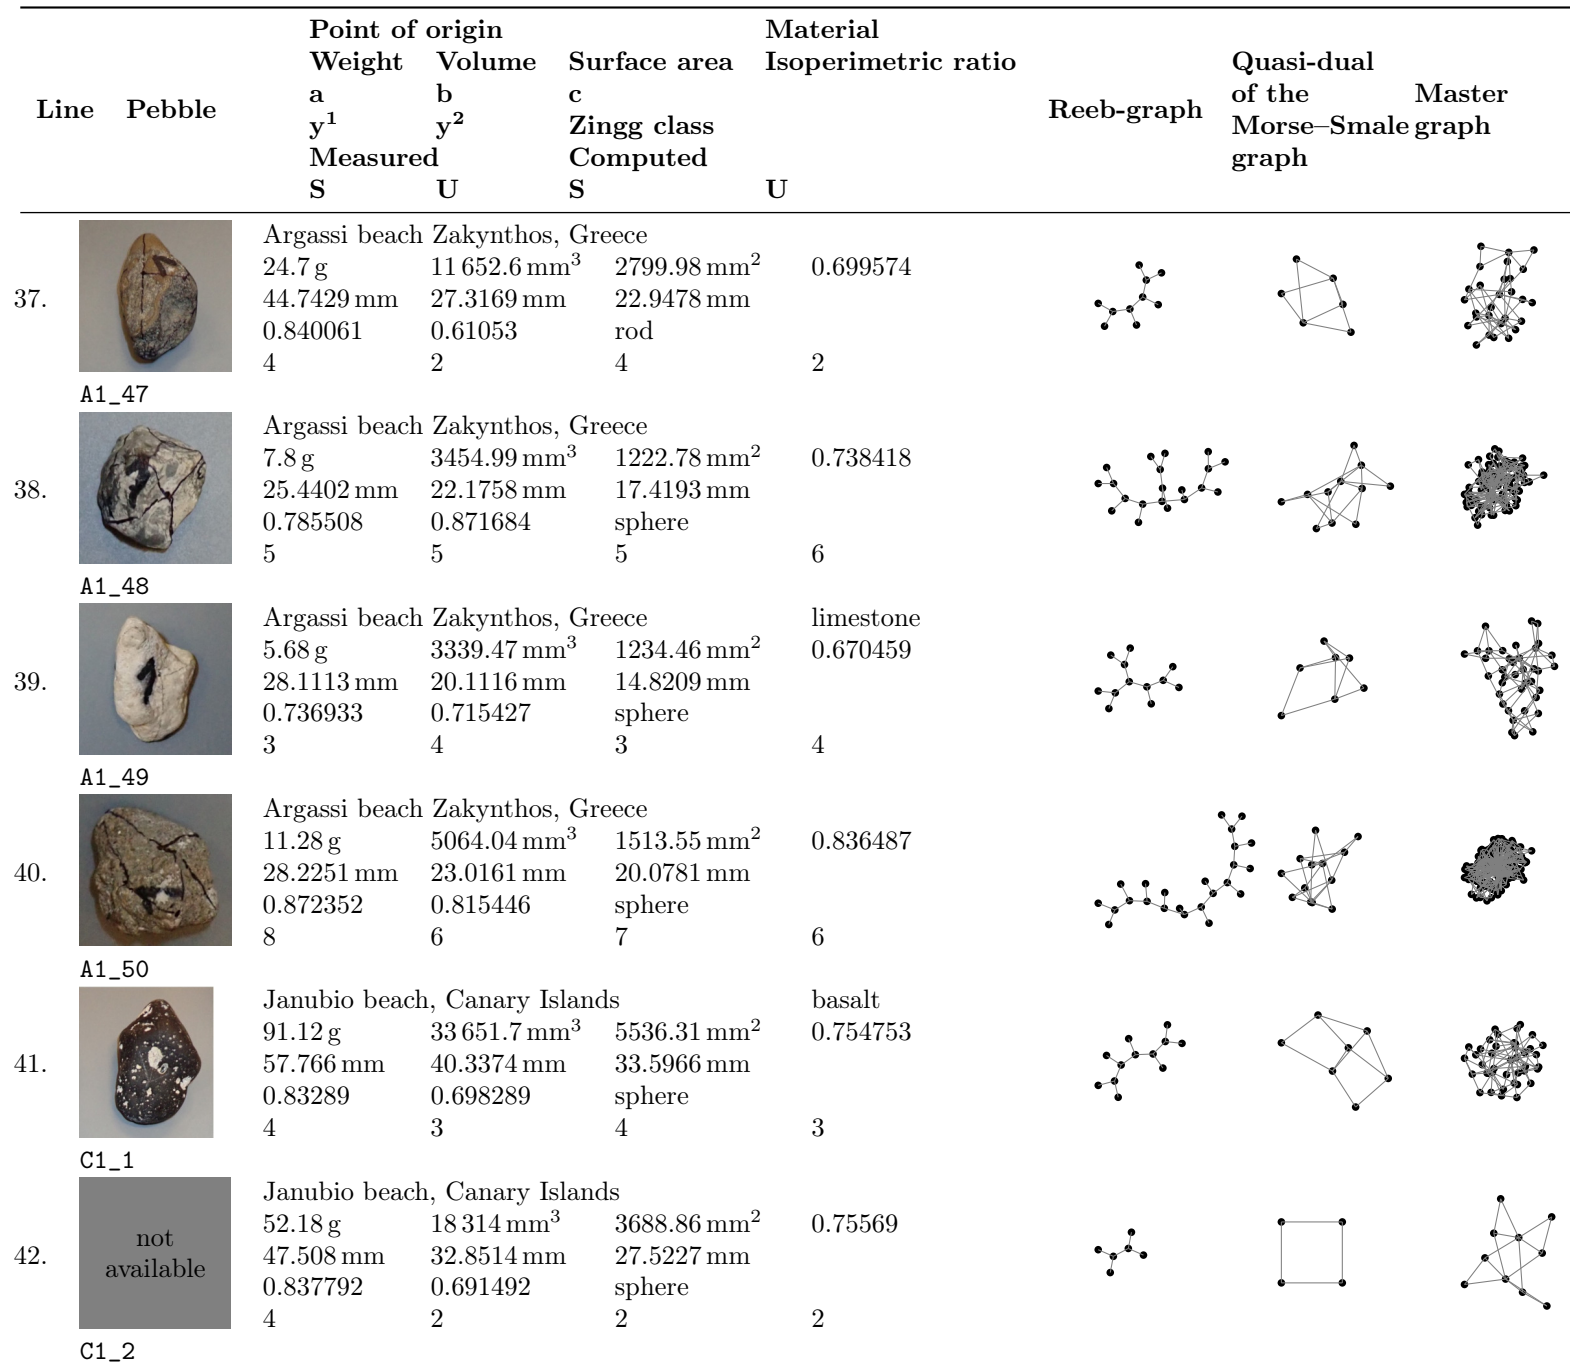   | 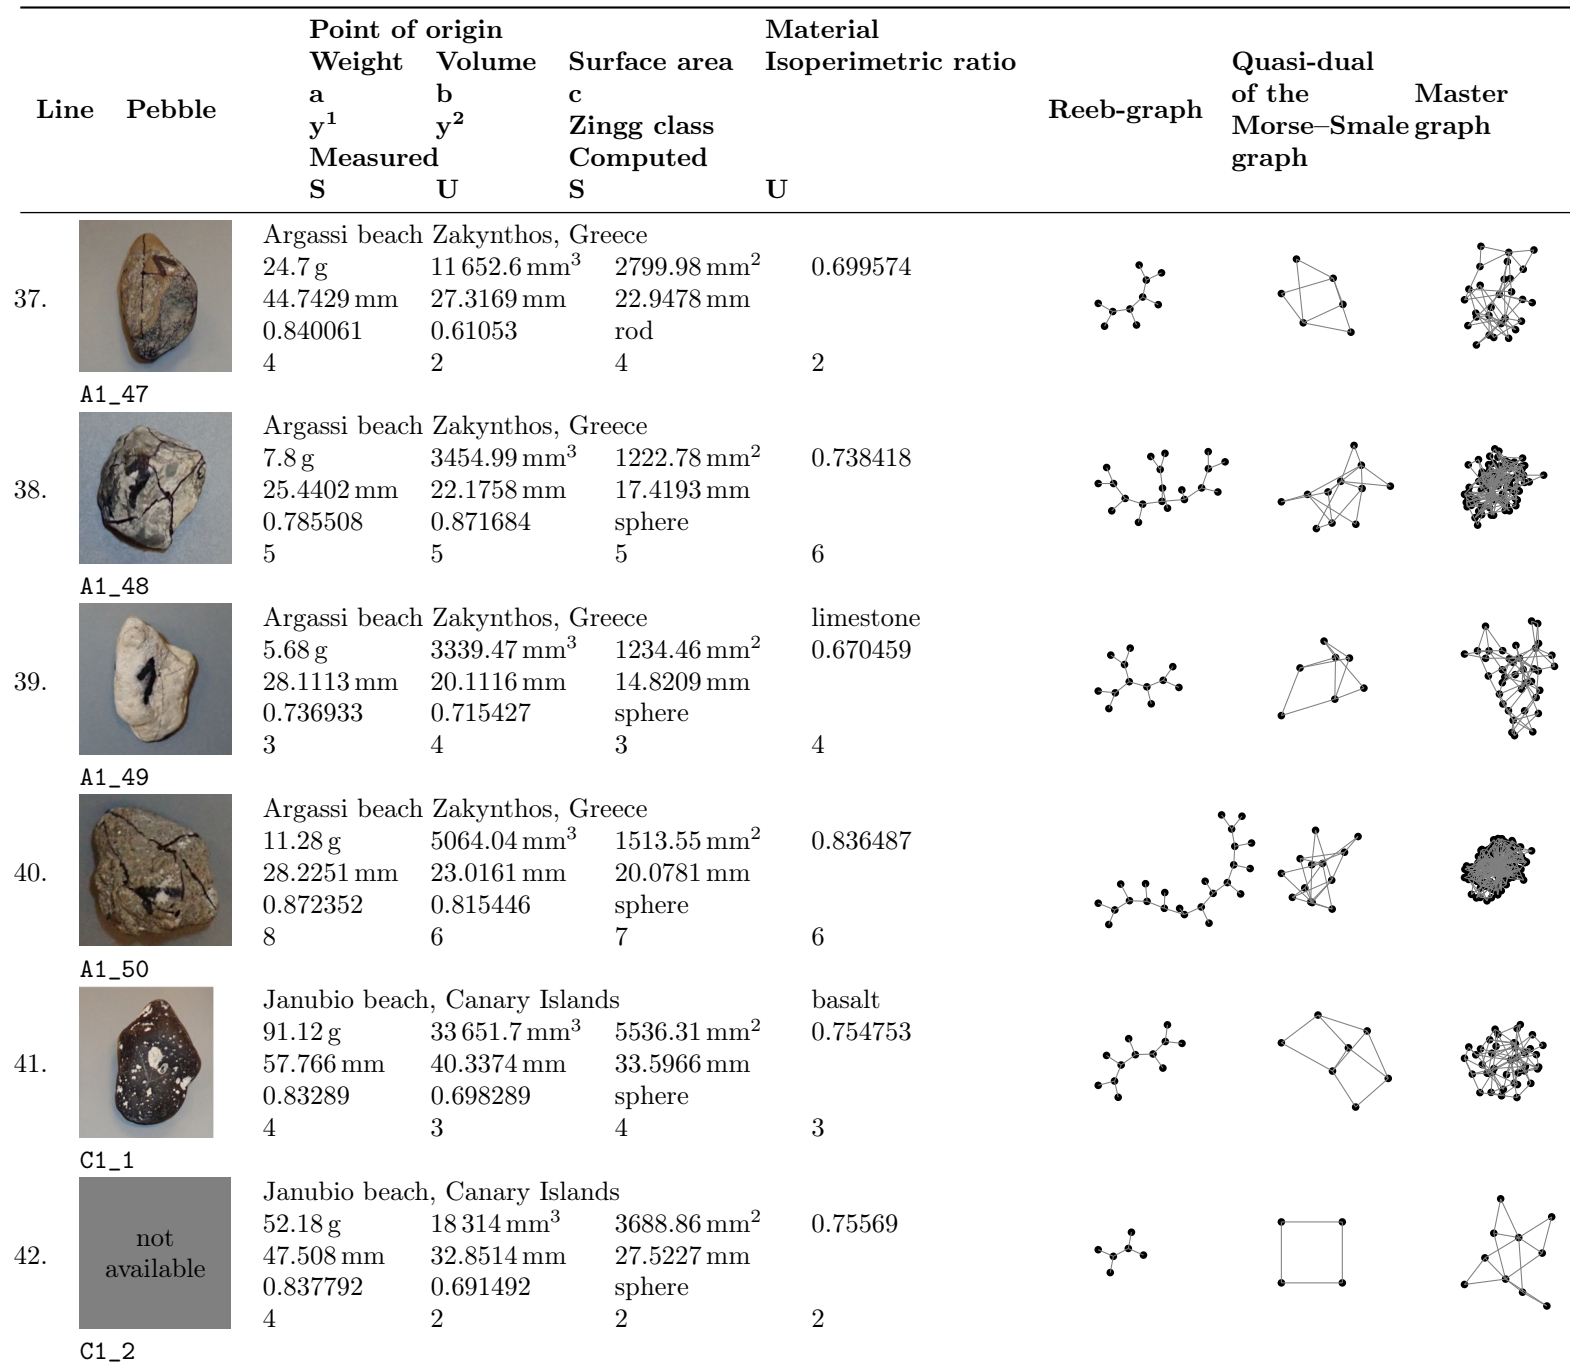   |
|      |                                                                                     | 7.8 g                                | 3454.99 mm <sup>3</sup>  |                                                      |                                      |                                                                                       |                                                                                       |                                                                                       |
|      |                                                                                     | 25.4402 mm                           | 22.1758 mm               |                                                      |                                      |                                                                                       |                                                                                       |                                                                                       |
|      |                                                                                     | 0.785508                             | 0.871684                 |                                                      |                                      |                                                                                       |                                                                                       |                                                                                       |
|      | A1_48                                                                               | 5                                    | 5                        |                                                      |                                      |                                                                                       |                                                                                       |                                                                                       |
| 39.  | 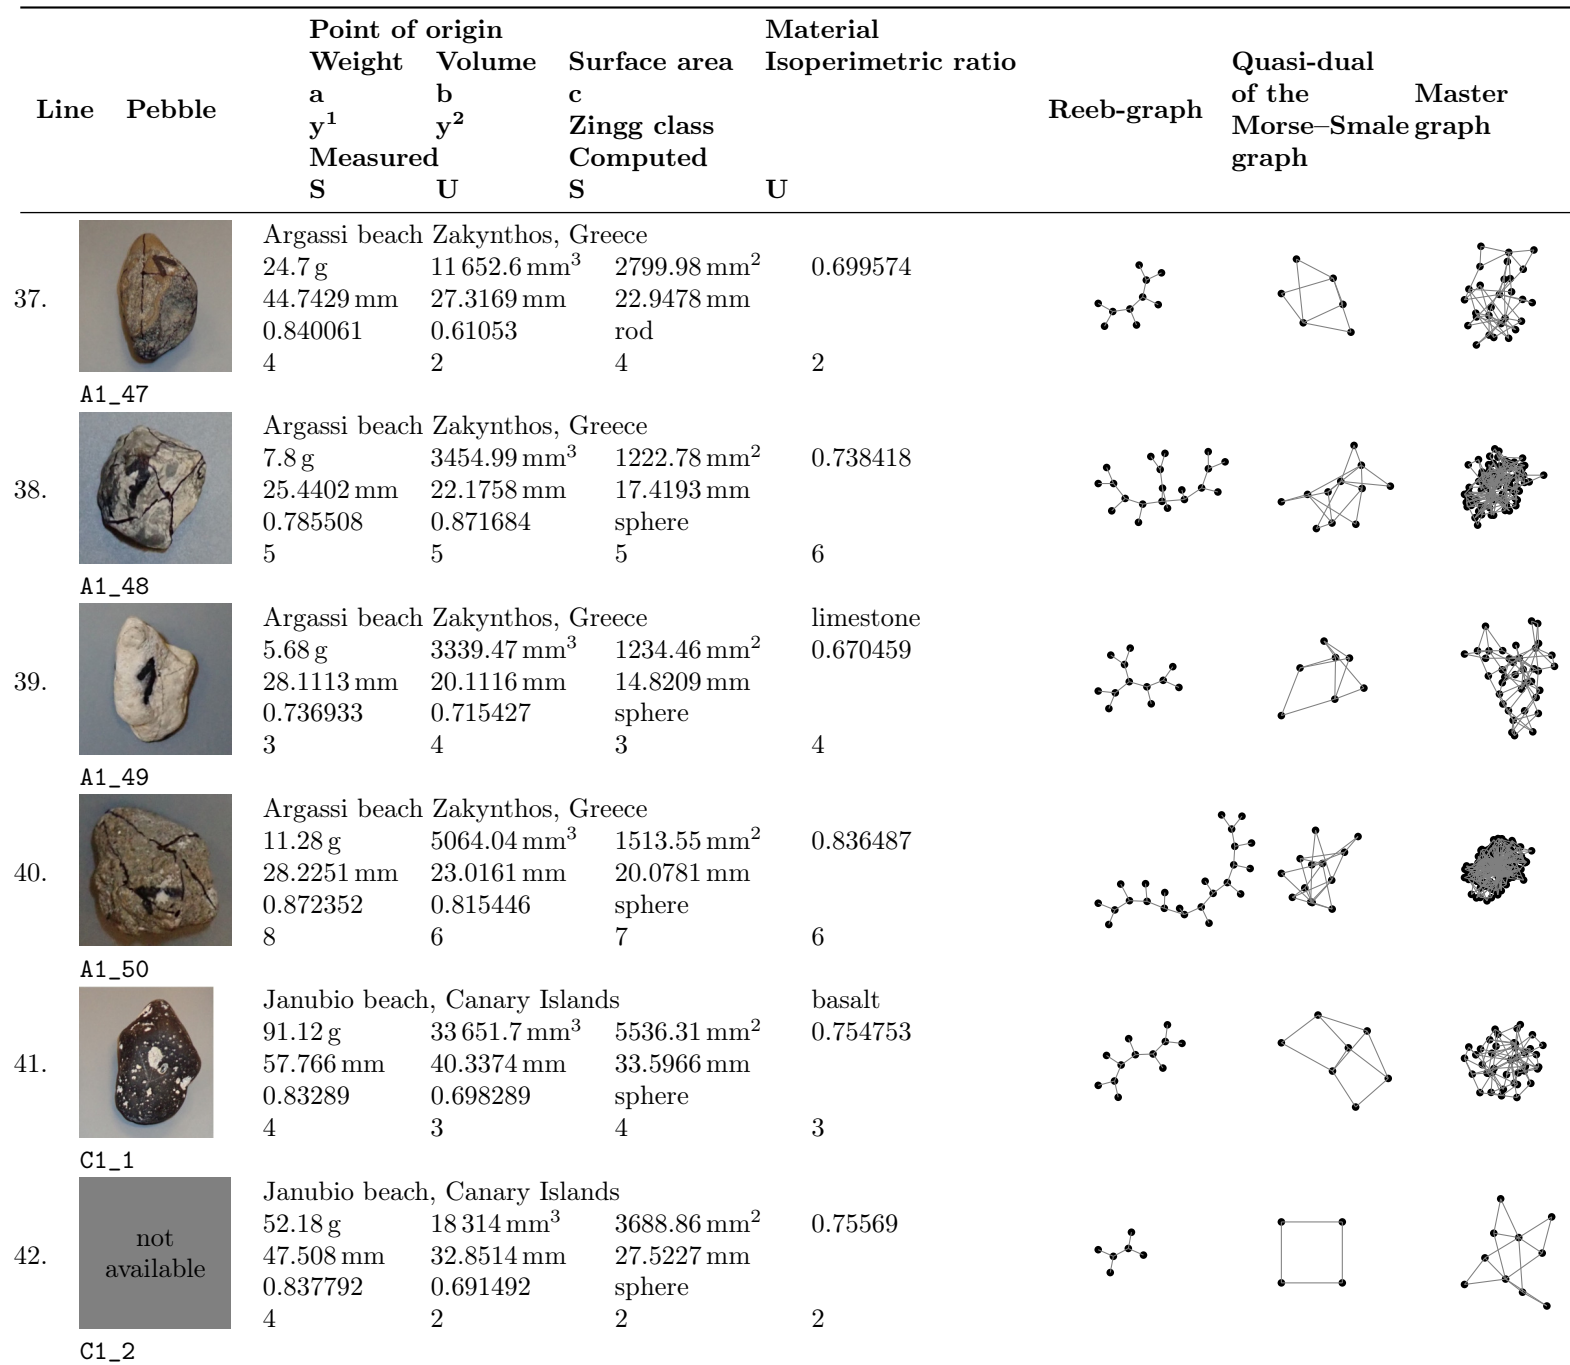   | Argassi beach Zakynthos, Greece      |                          | 1234.46 mm <sup>2</sup><br>14.8209 mm<br>sphere<br>3 | limestone<br>0.670459<br>4           | 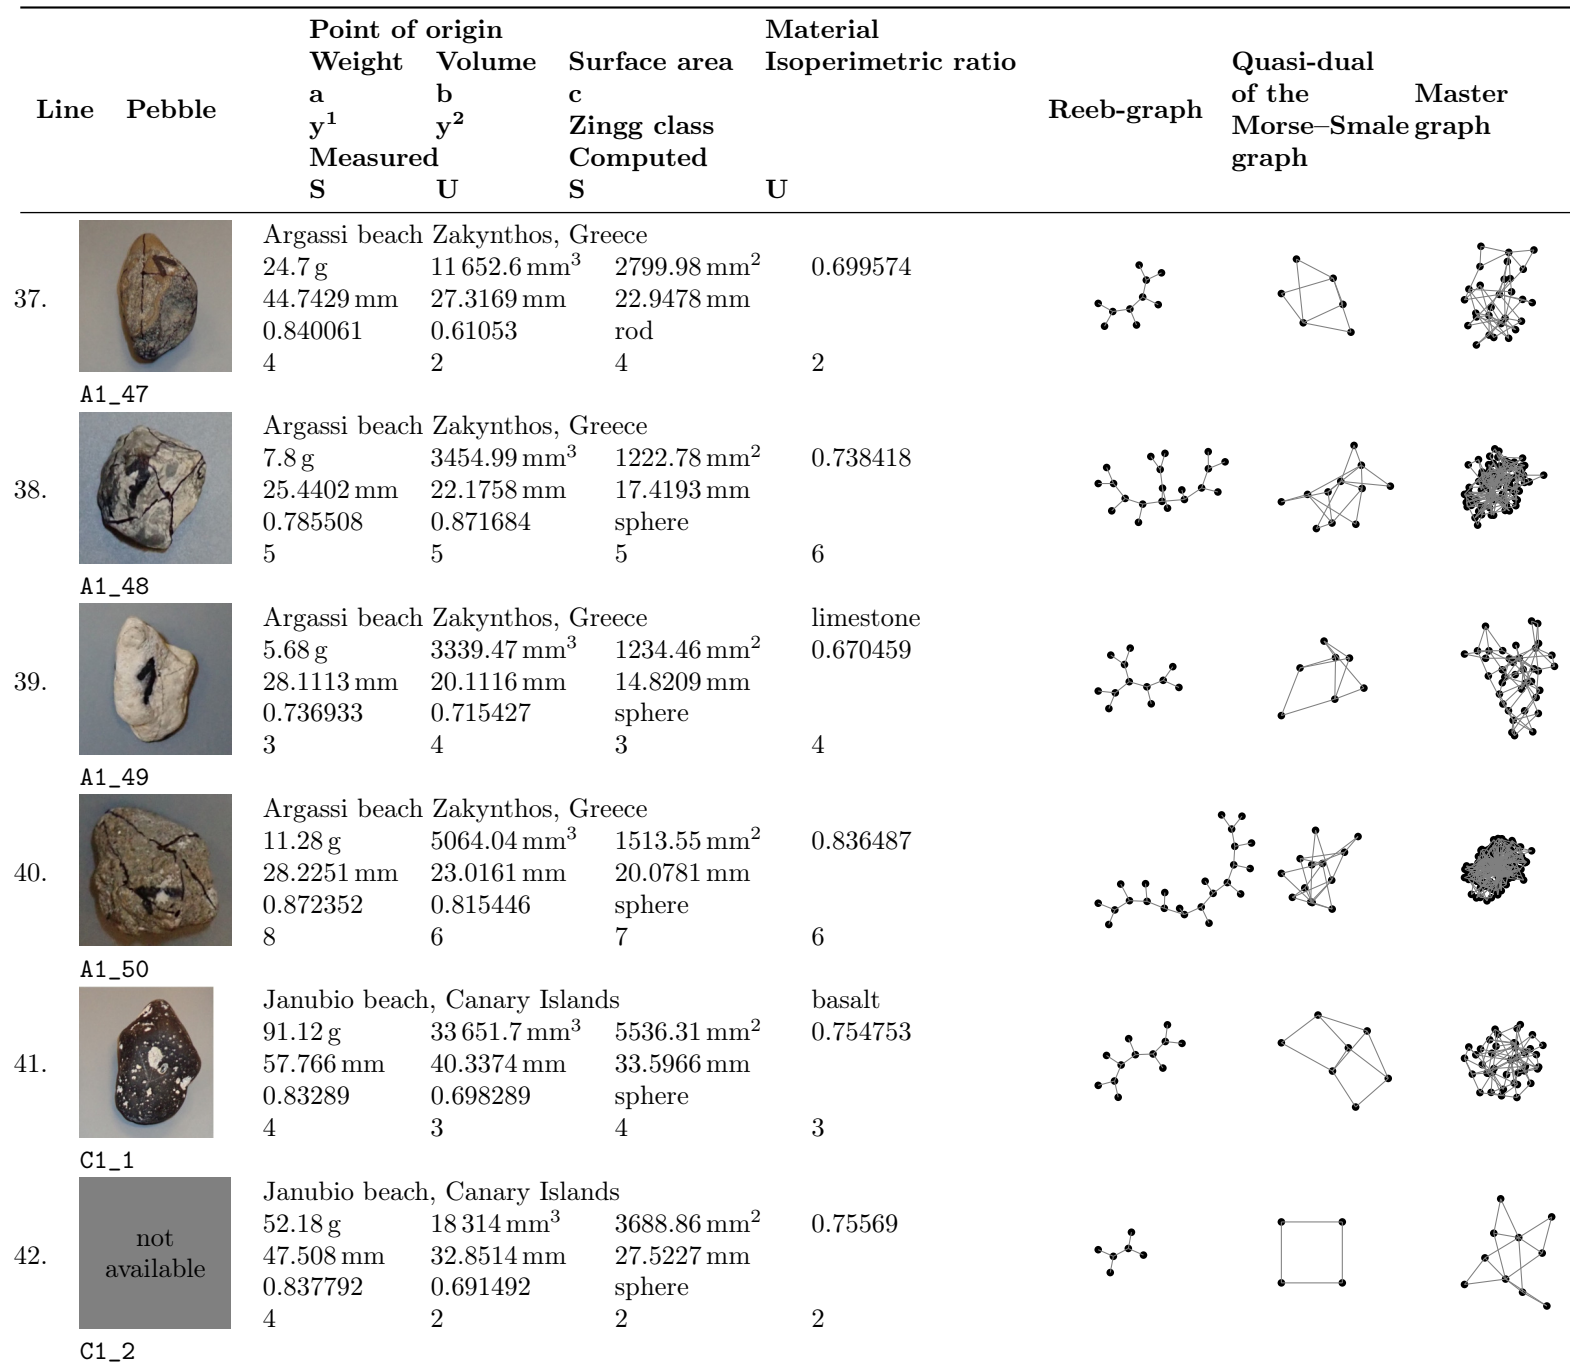   | 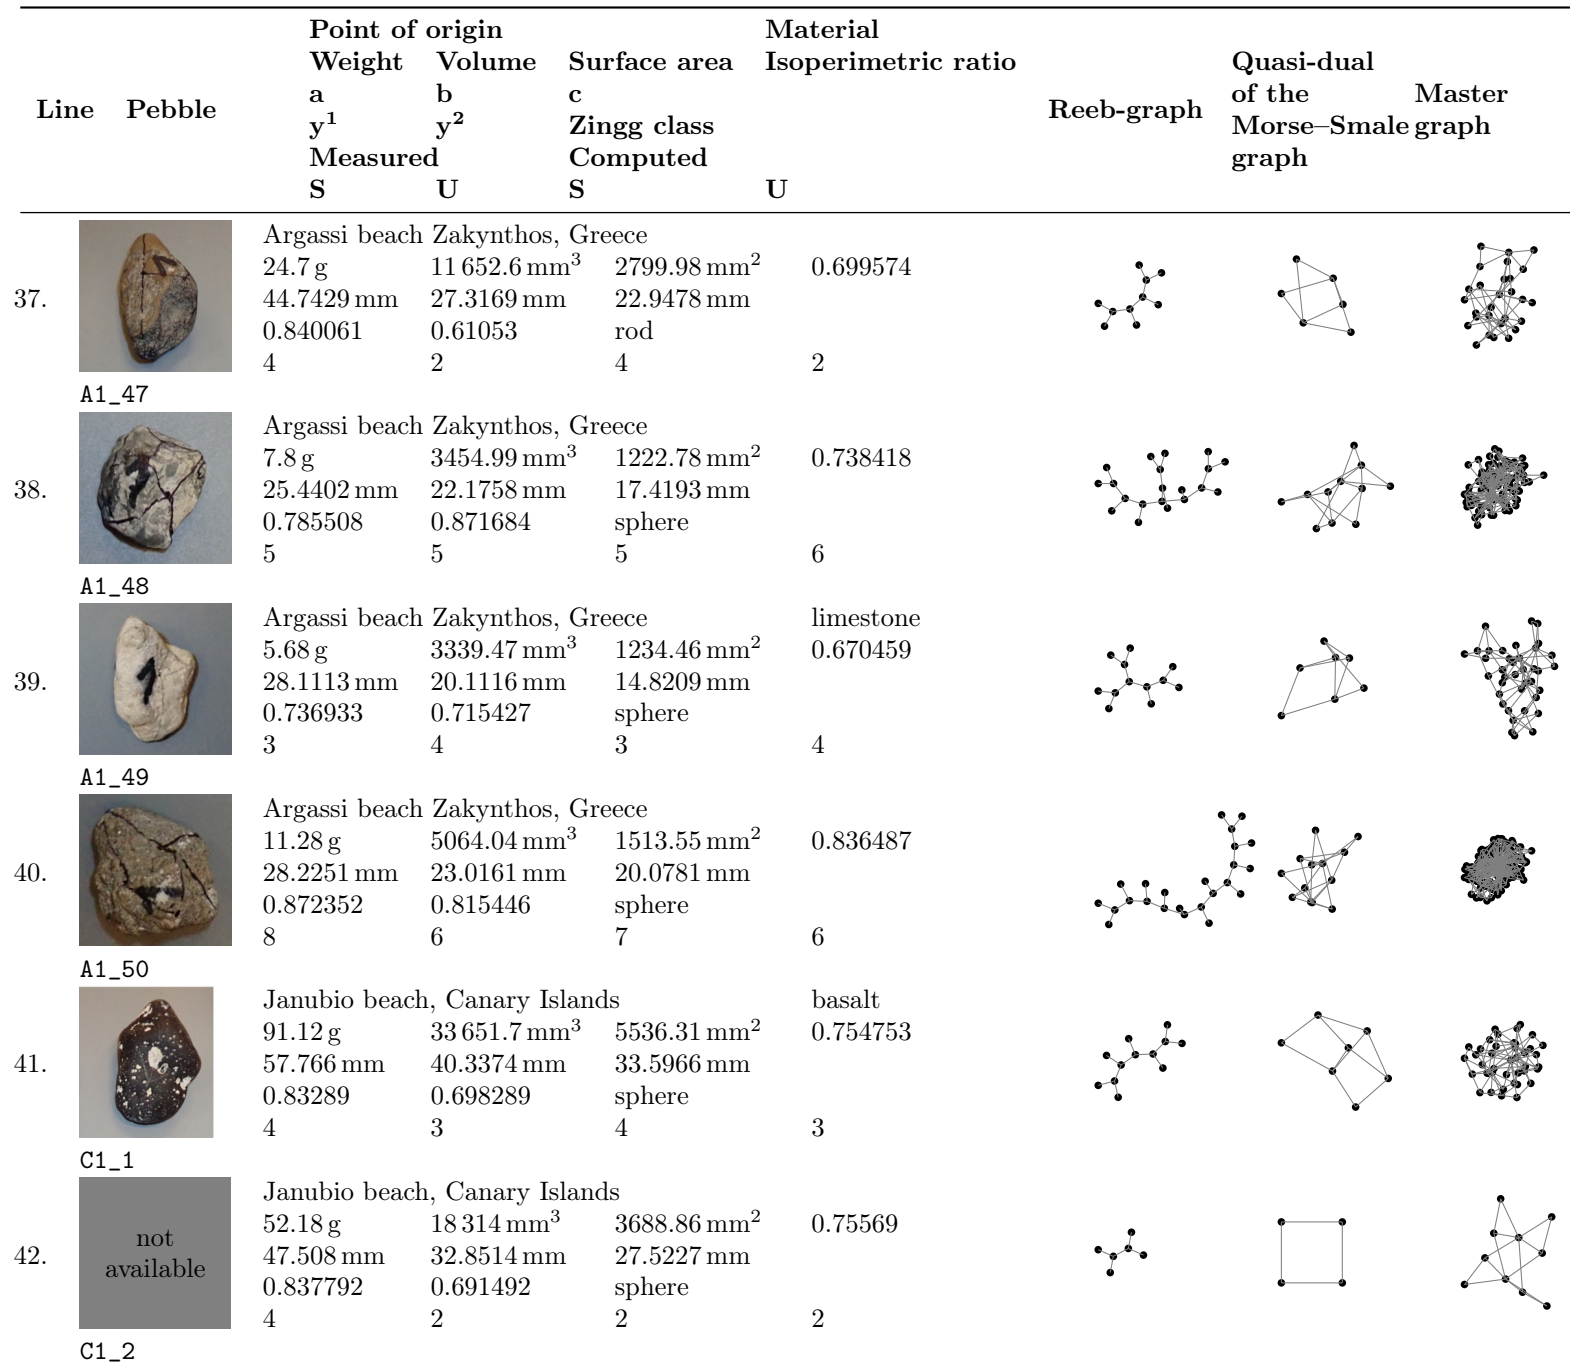   | 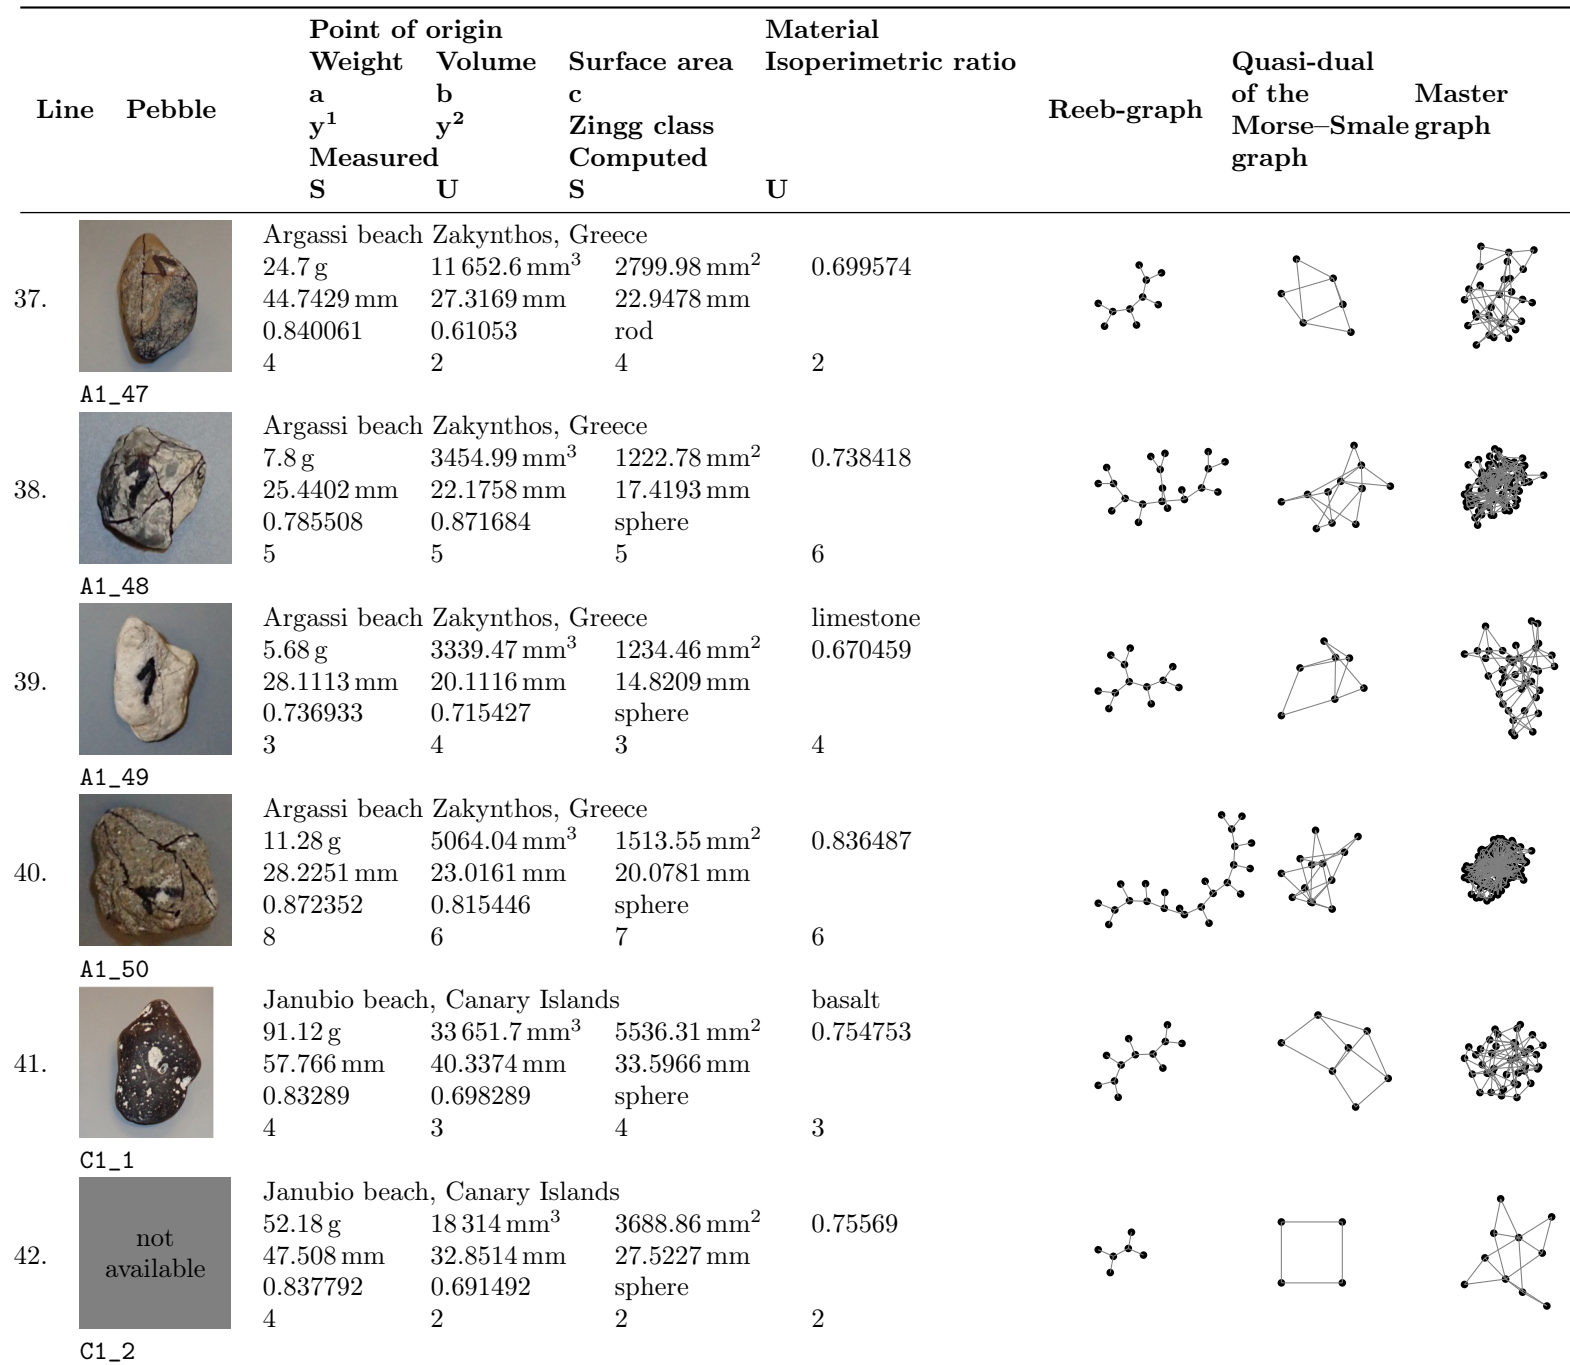   |
|      |                                                                                     | 5.68 g                               | 3339.47 mm <sup>3</sup>  |                                                      |                                      |                                                                                       |                                                                                       |                                                                                       |
|      |                                                                                     | 28.1113 mm                           | 20.1116 mm               |                                                      |                                      |                                                                                       |                                                                                       |                                                                                       |
|      |                                                                                     | 0.736933                             | 0.715427                 |                                                      |                                      |                                                                                       |                                                                                       |                                                                                       |
|      | A1_49                                                                               | 3                                    | 4                        |                                                      |                                      |                                                                                       |                                                                                       |                                                                                       |
| 40.  | 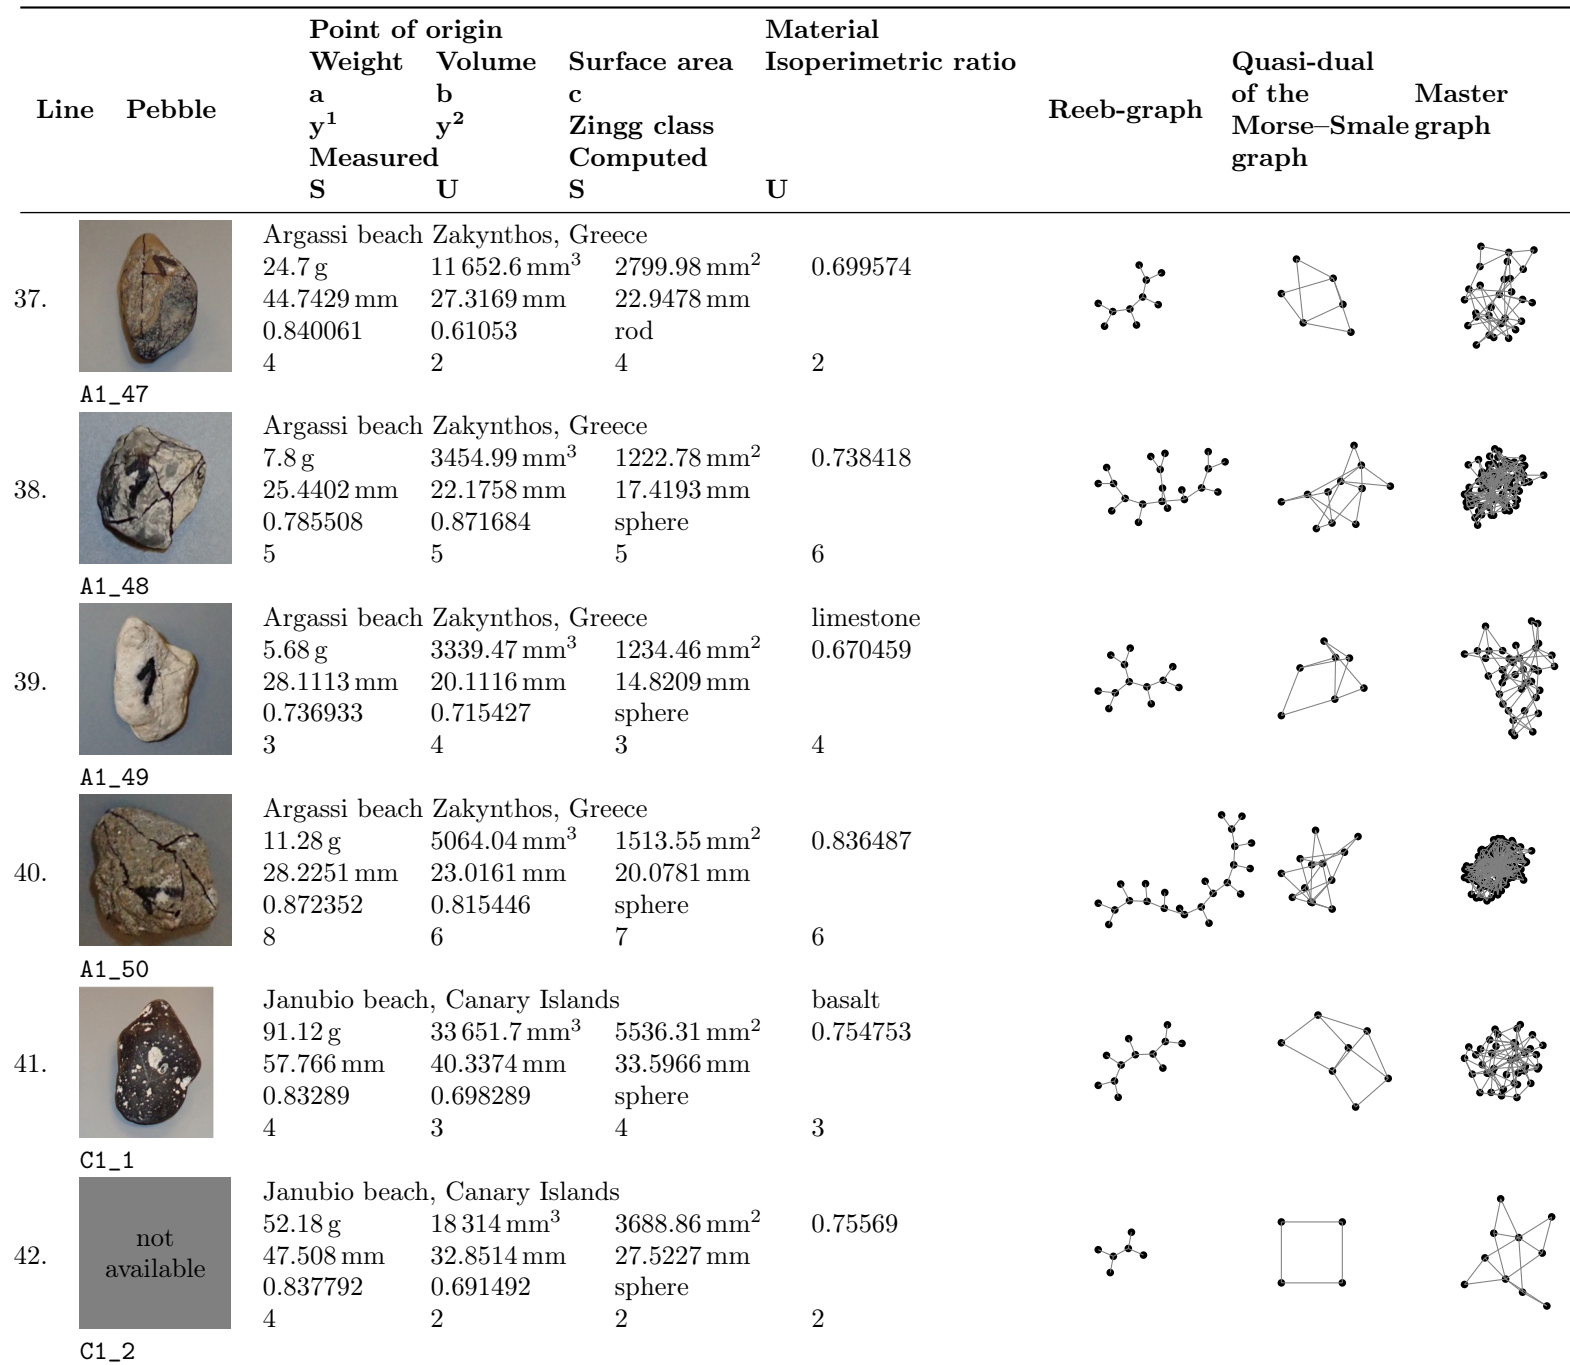  | Argassi beach Zakynthos, Greece      |                          | 1513.55 mm <sup>2</sup><br>20.0781 mm<br>sphere<br>7 | 0.836487<br>6                        | 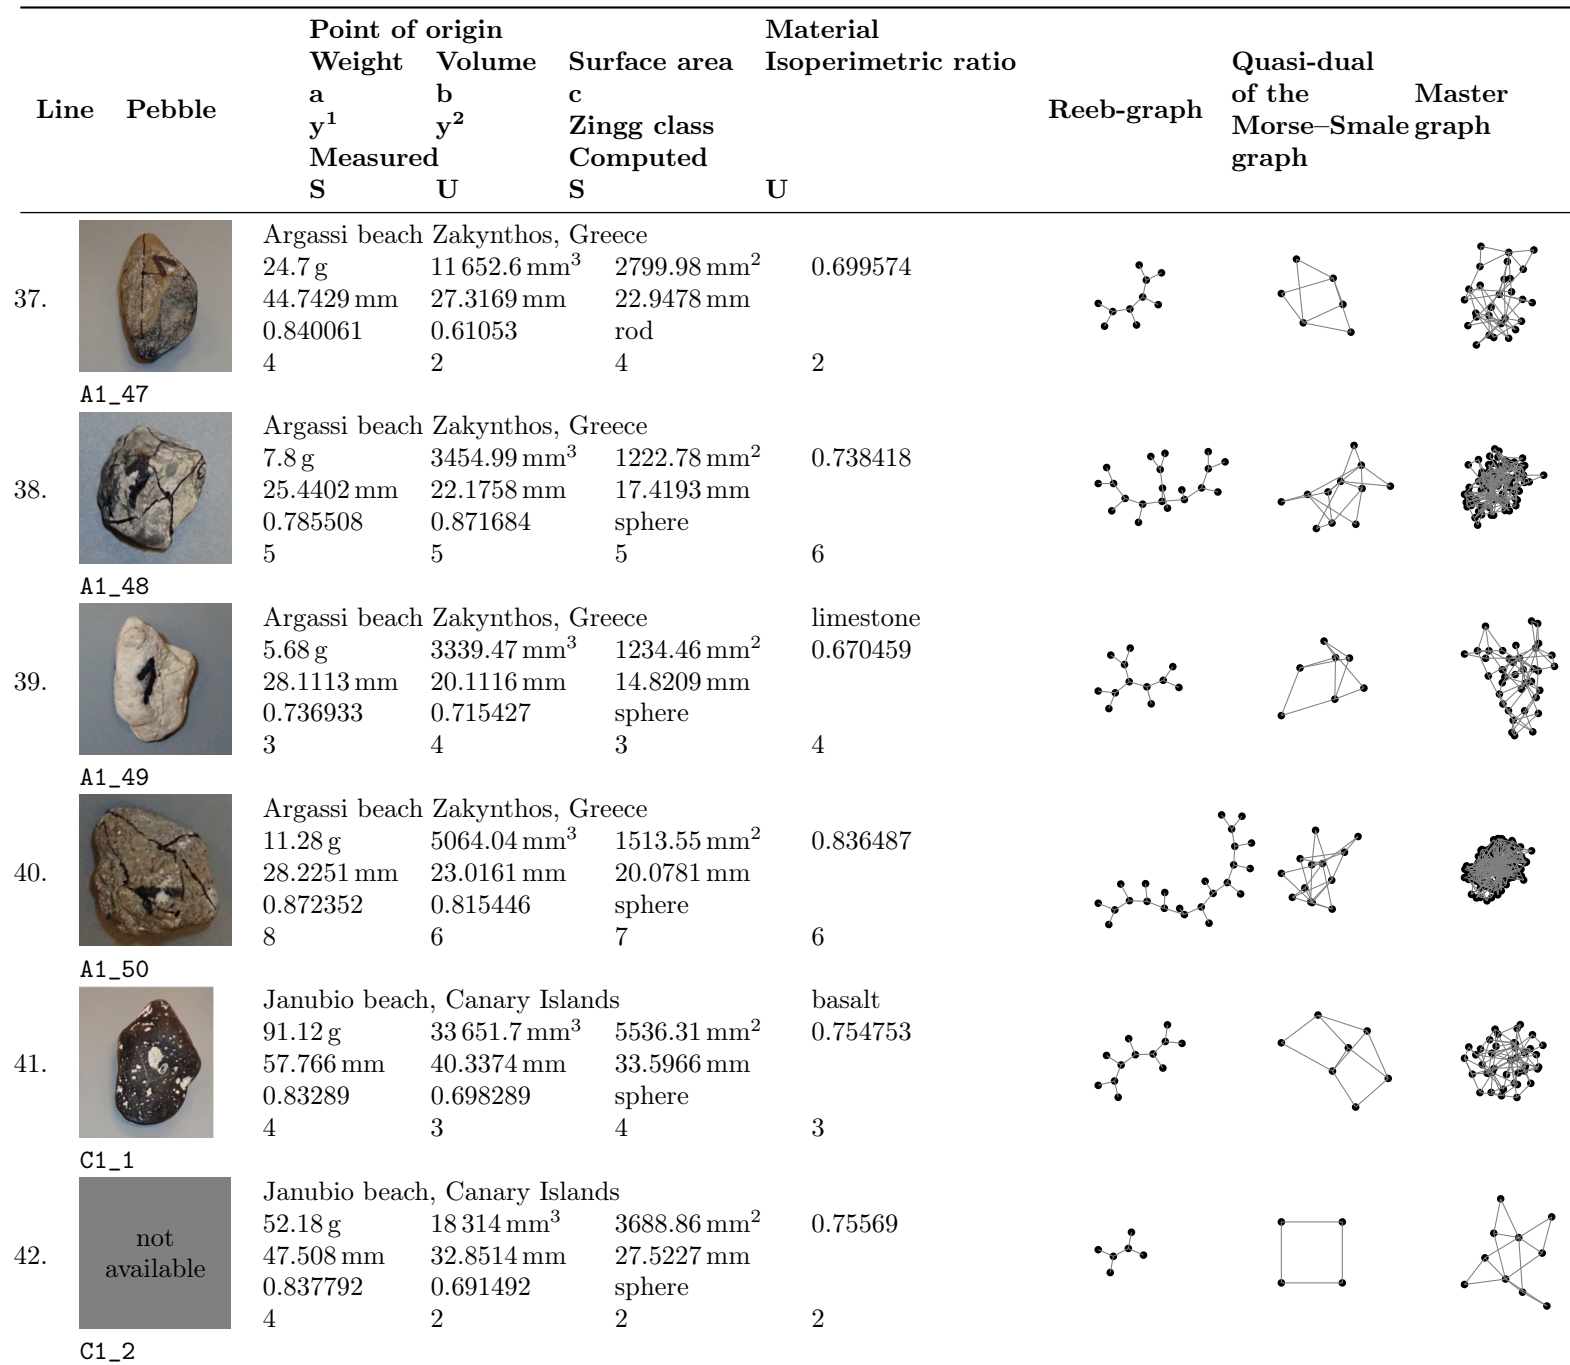  | 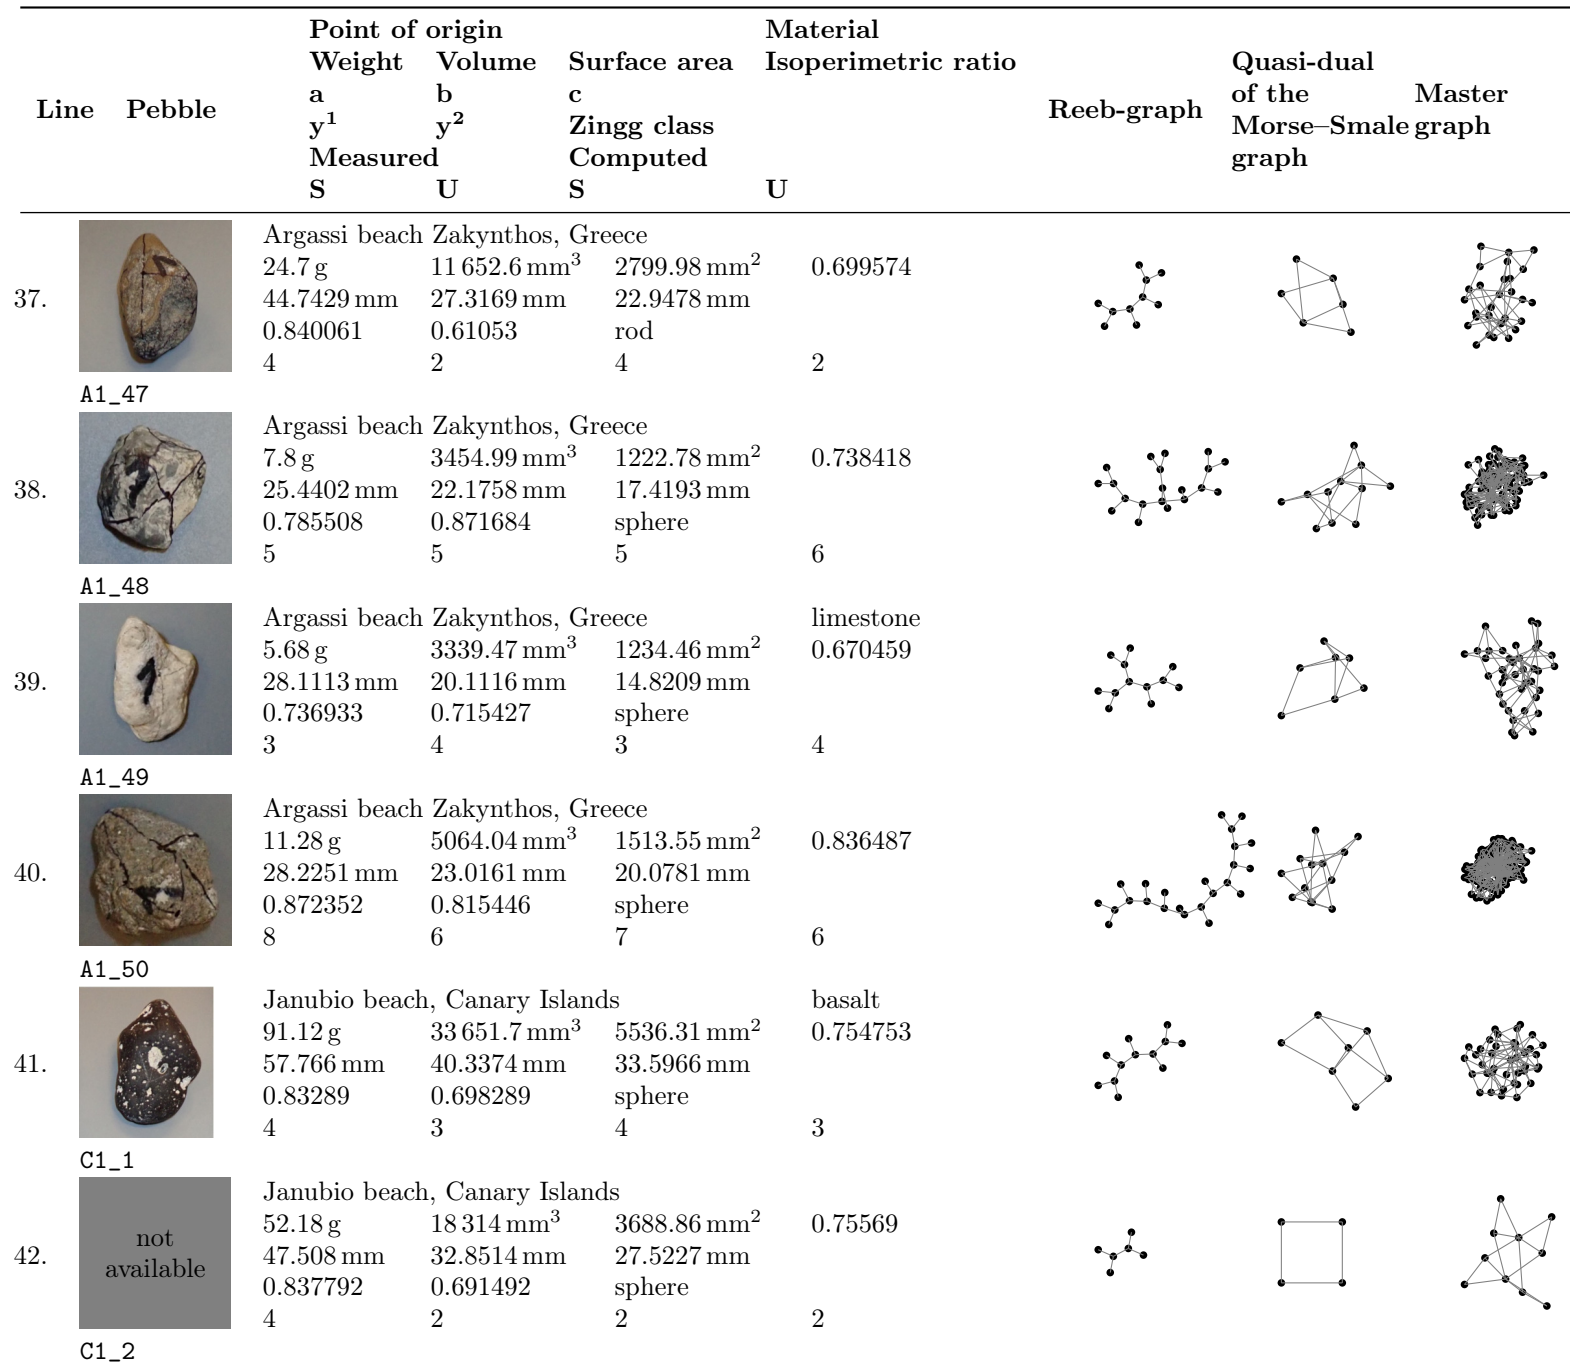  | 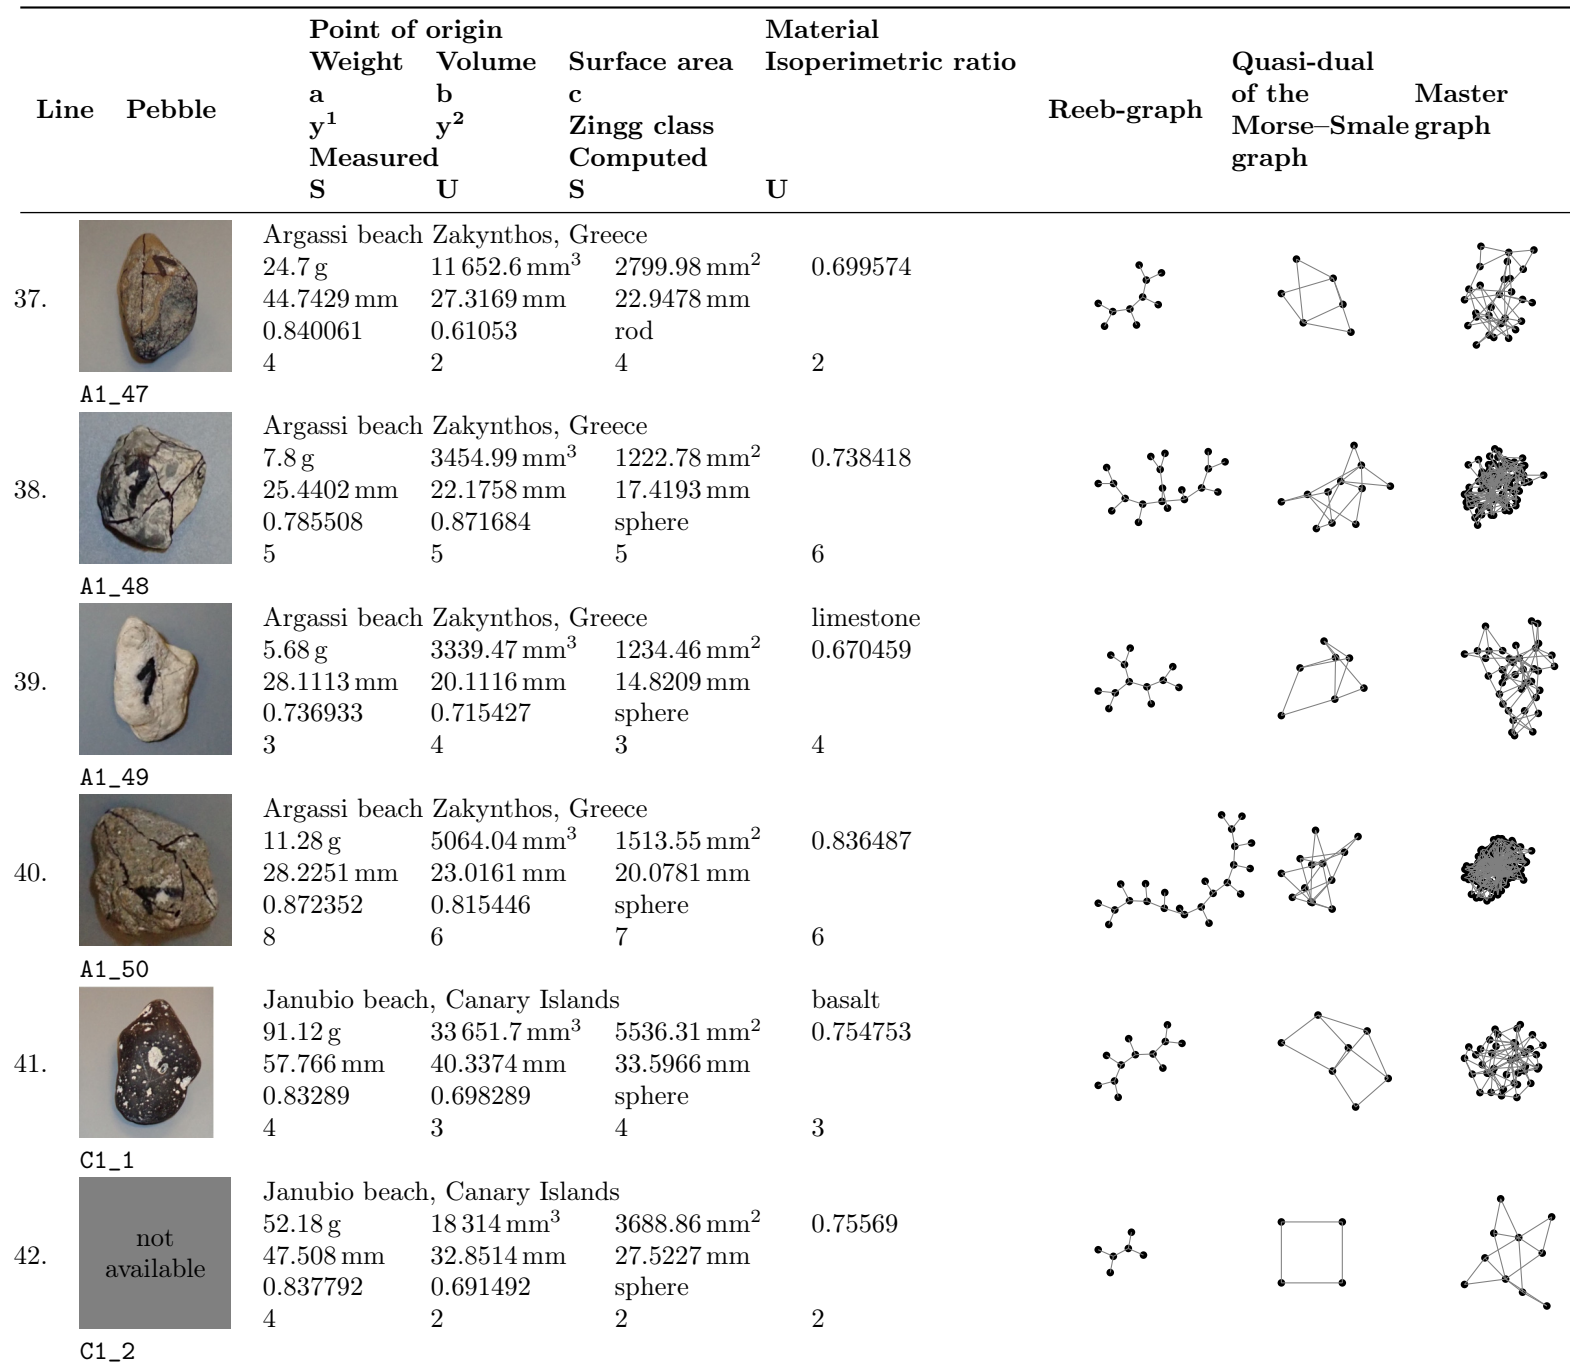  |
|      |                                                                                     | 11.28 g                              | 5064.04 mm <sup>3</sup>  |                                                      |                                      |                                                                                       |                                                                                       |                                                                                       |
|      |                                                                                     | 28.2251 mm                           | 23.0161 mm               |                                                      |                                      |                                                                                       |                                                                                       |                                                                                       |
|      |                                                                                     | 0.872352                             | 0.815446                 |                                                      |                                      |                                                                                       |                                                                                       |                                                                                       |
|      | A1_50                                                                               | 8                                    | 6                        |                                                      |                                      |                                                                                       |                                                                                       |                                                                                       |
| 41.  | 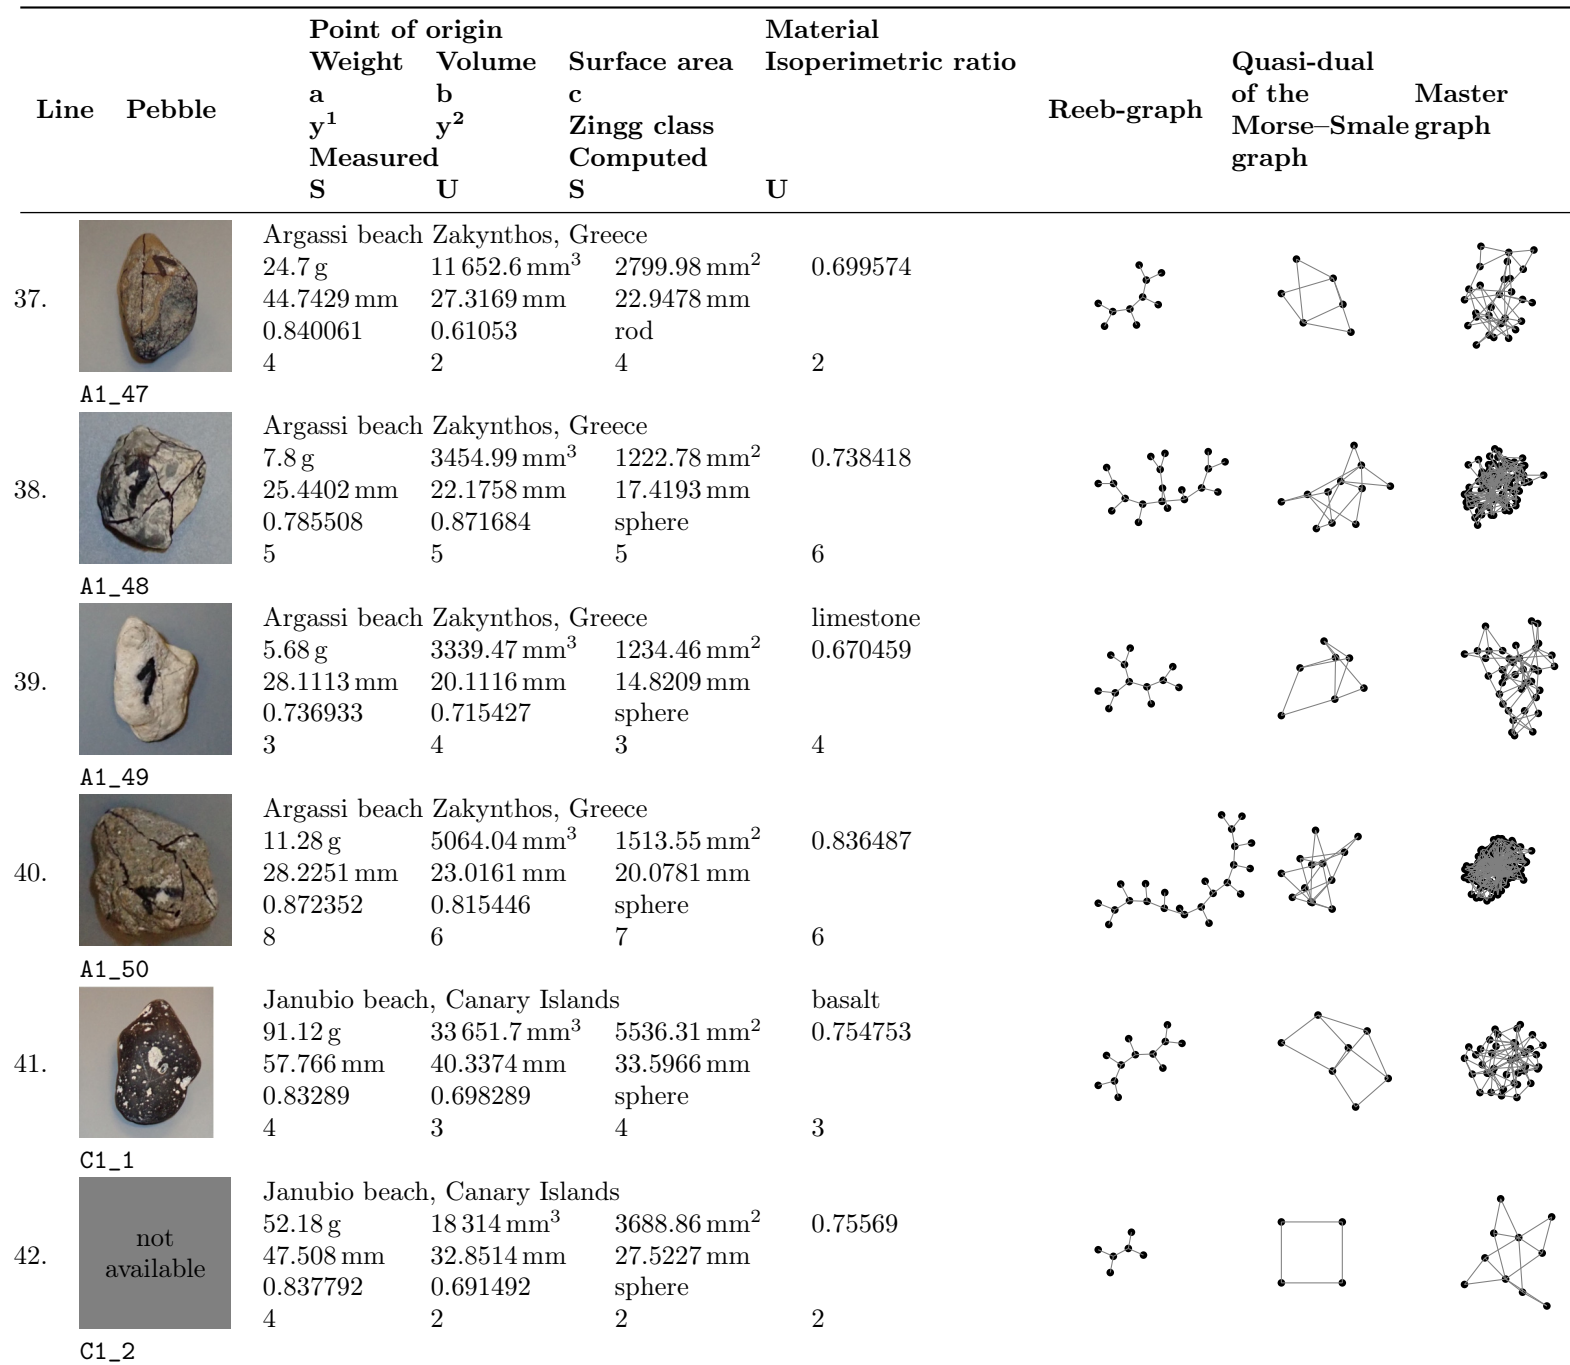 | Janubio beach, Canary Islands        |                          | 5536.31 mm <sup>2</sup><br>33.5966 mm<br>sphere<br>4 | basalt<br>0.754753<br>3              | 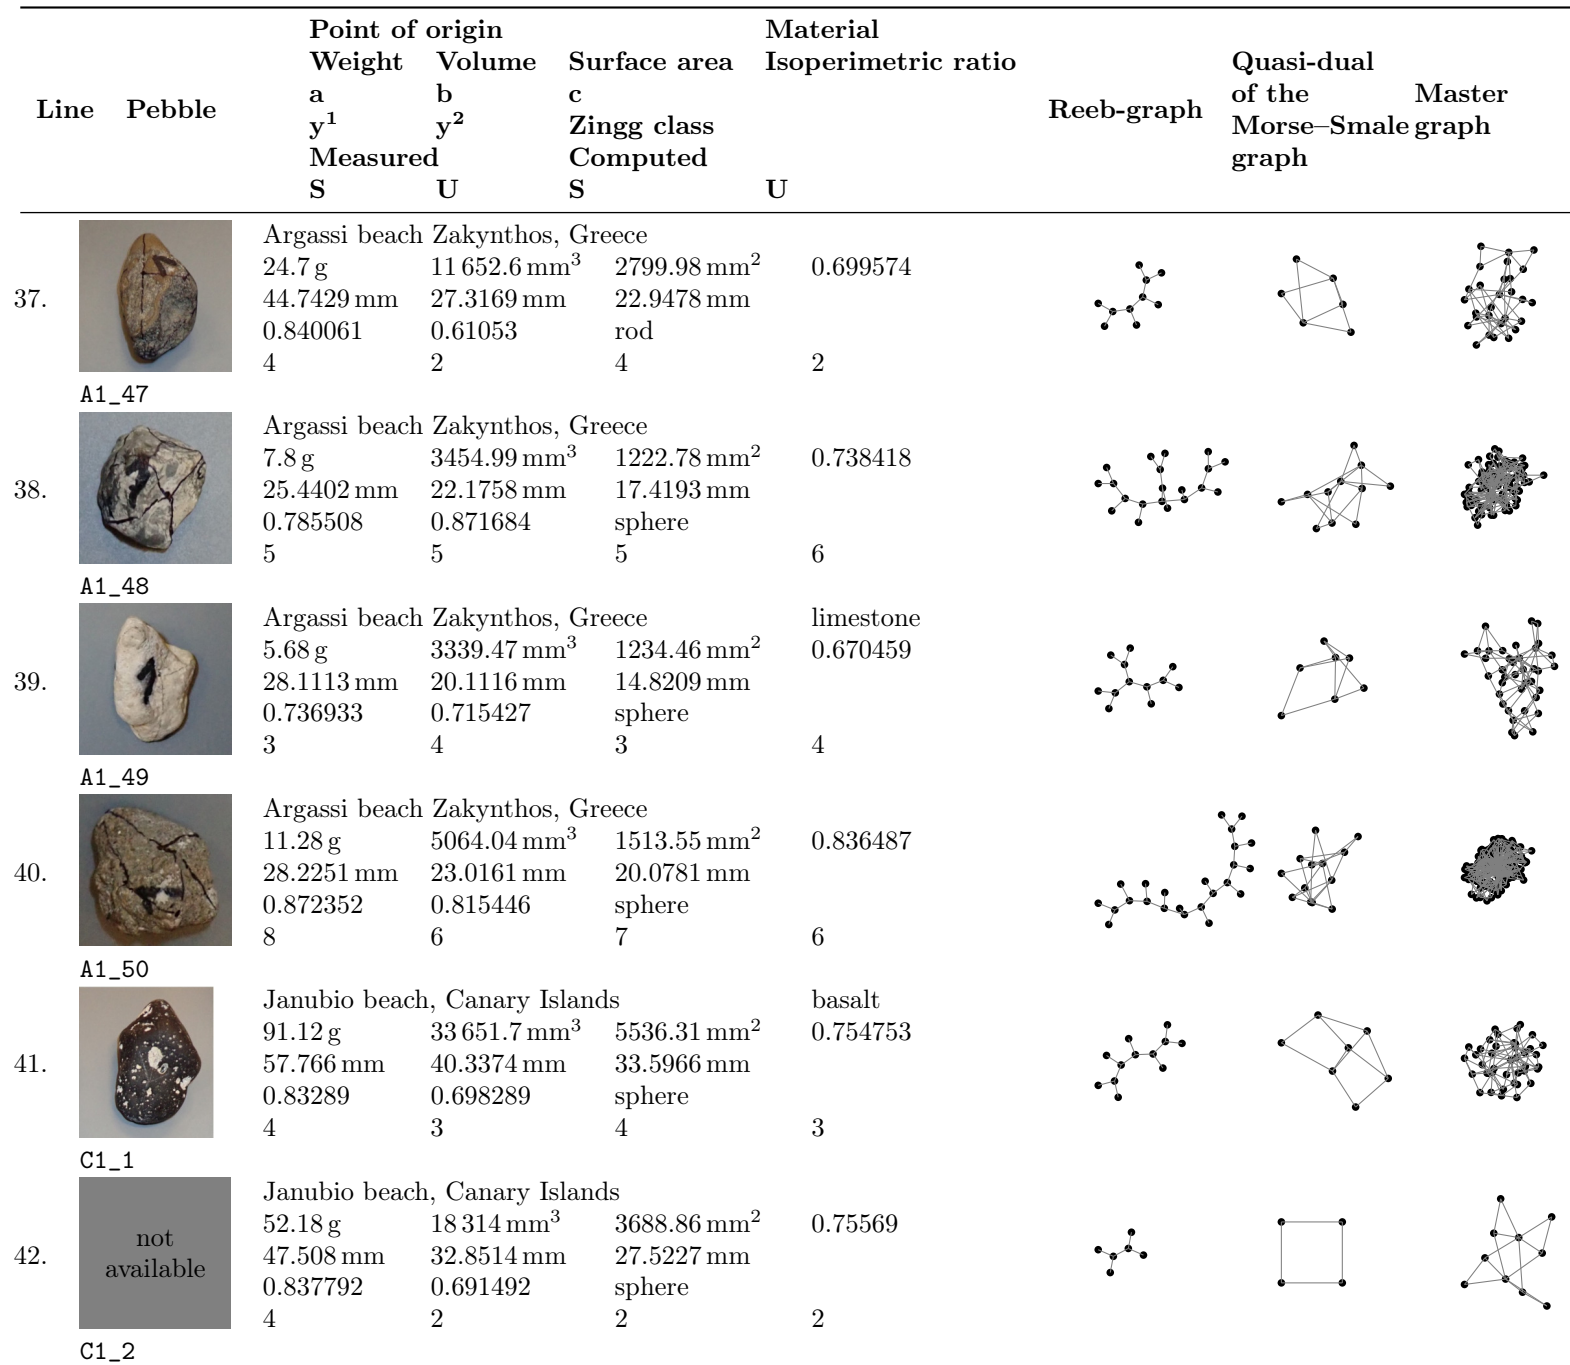 | 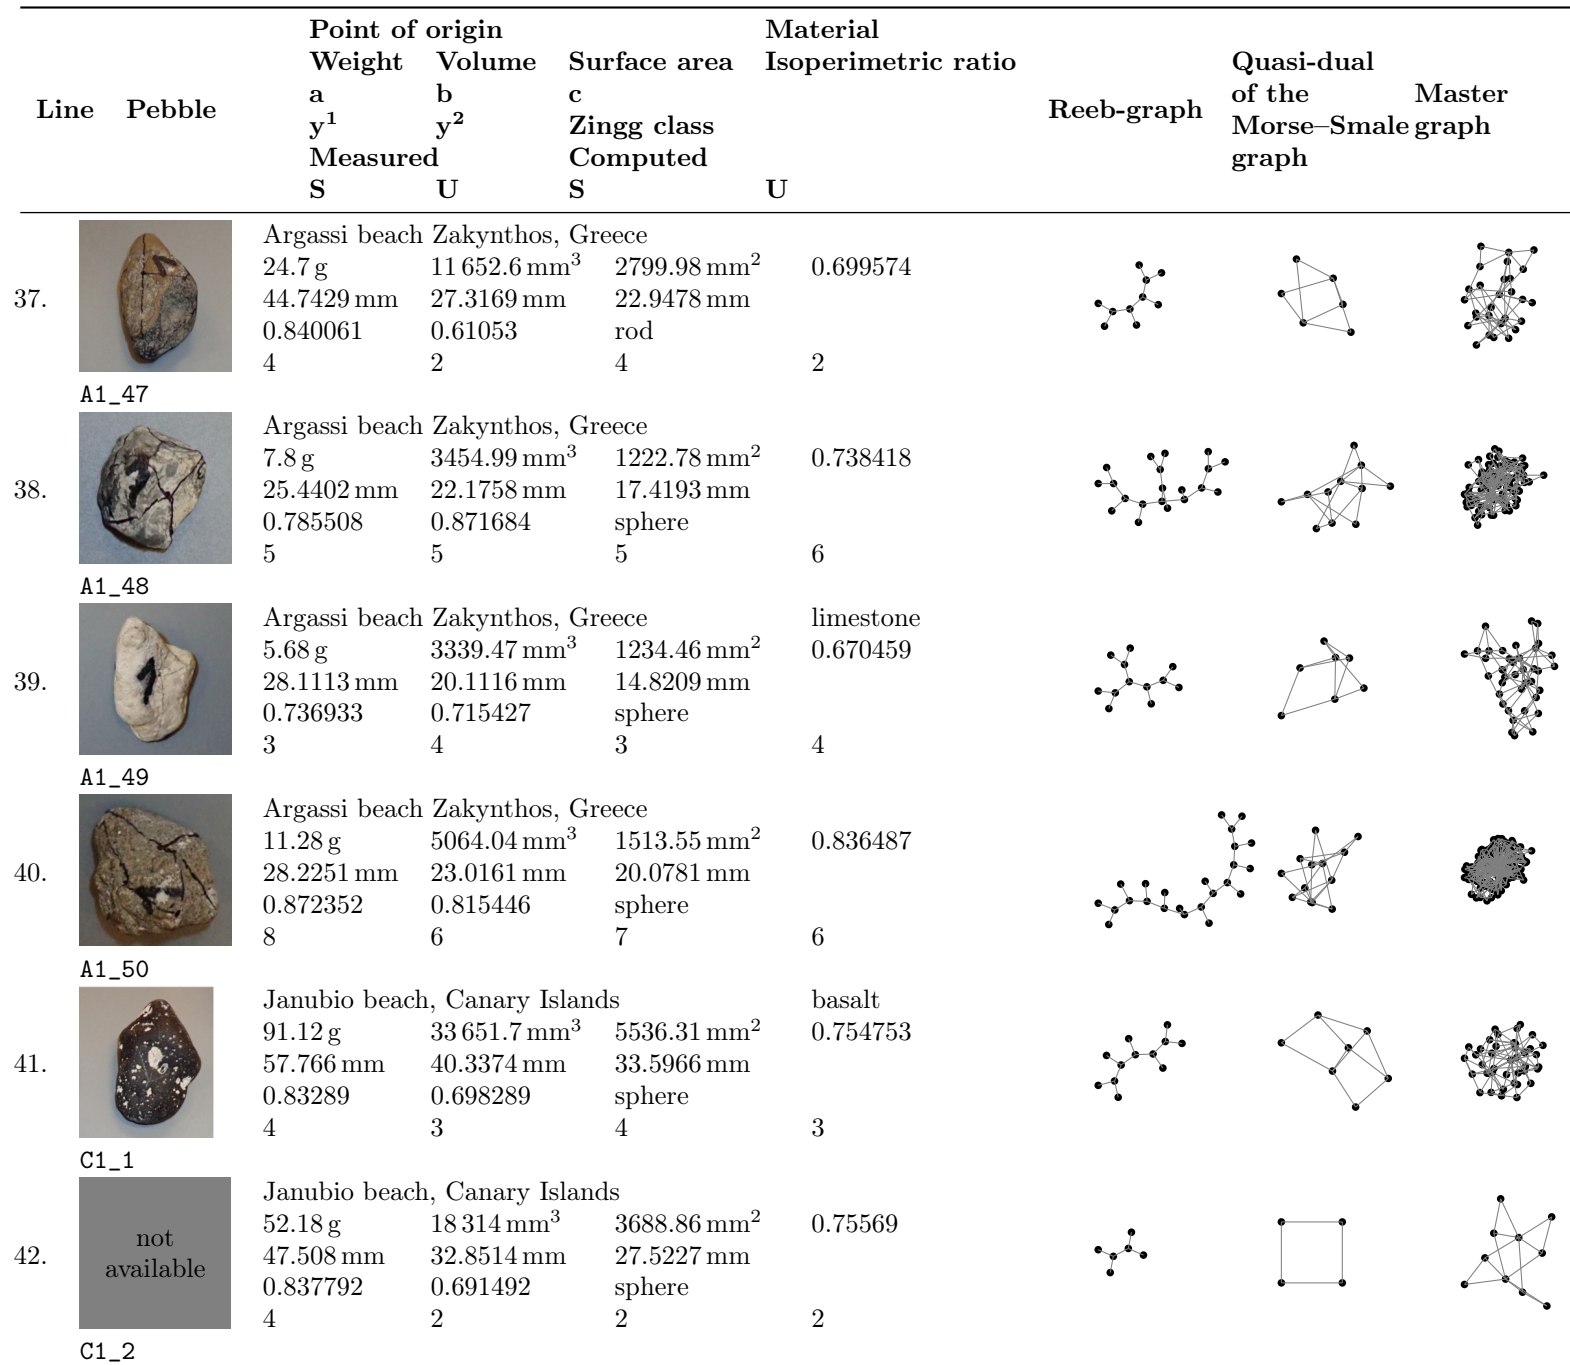 | 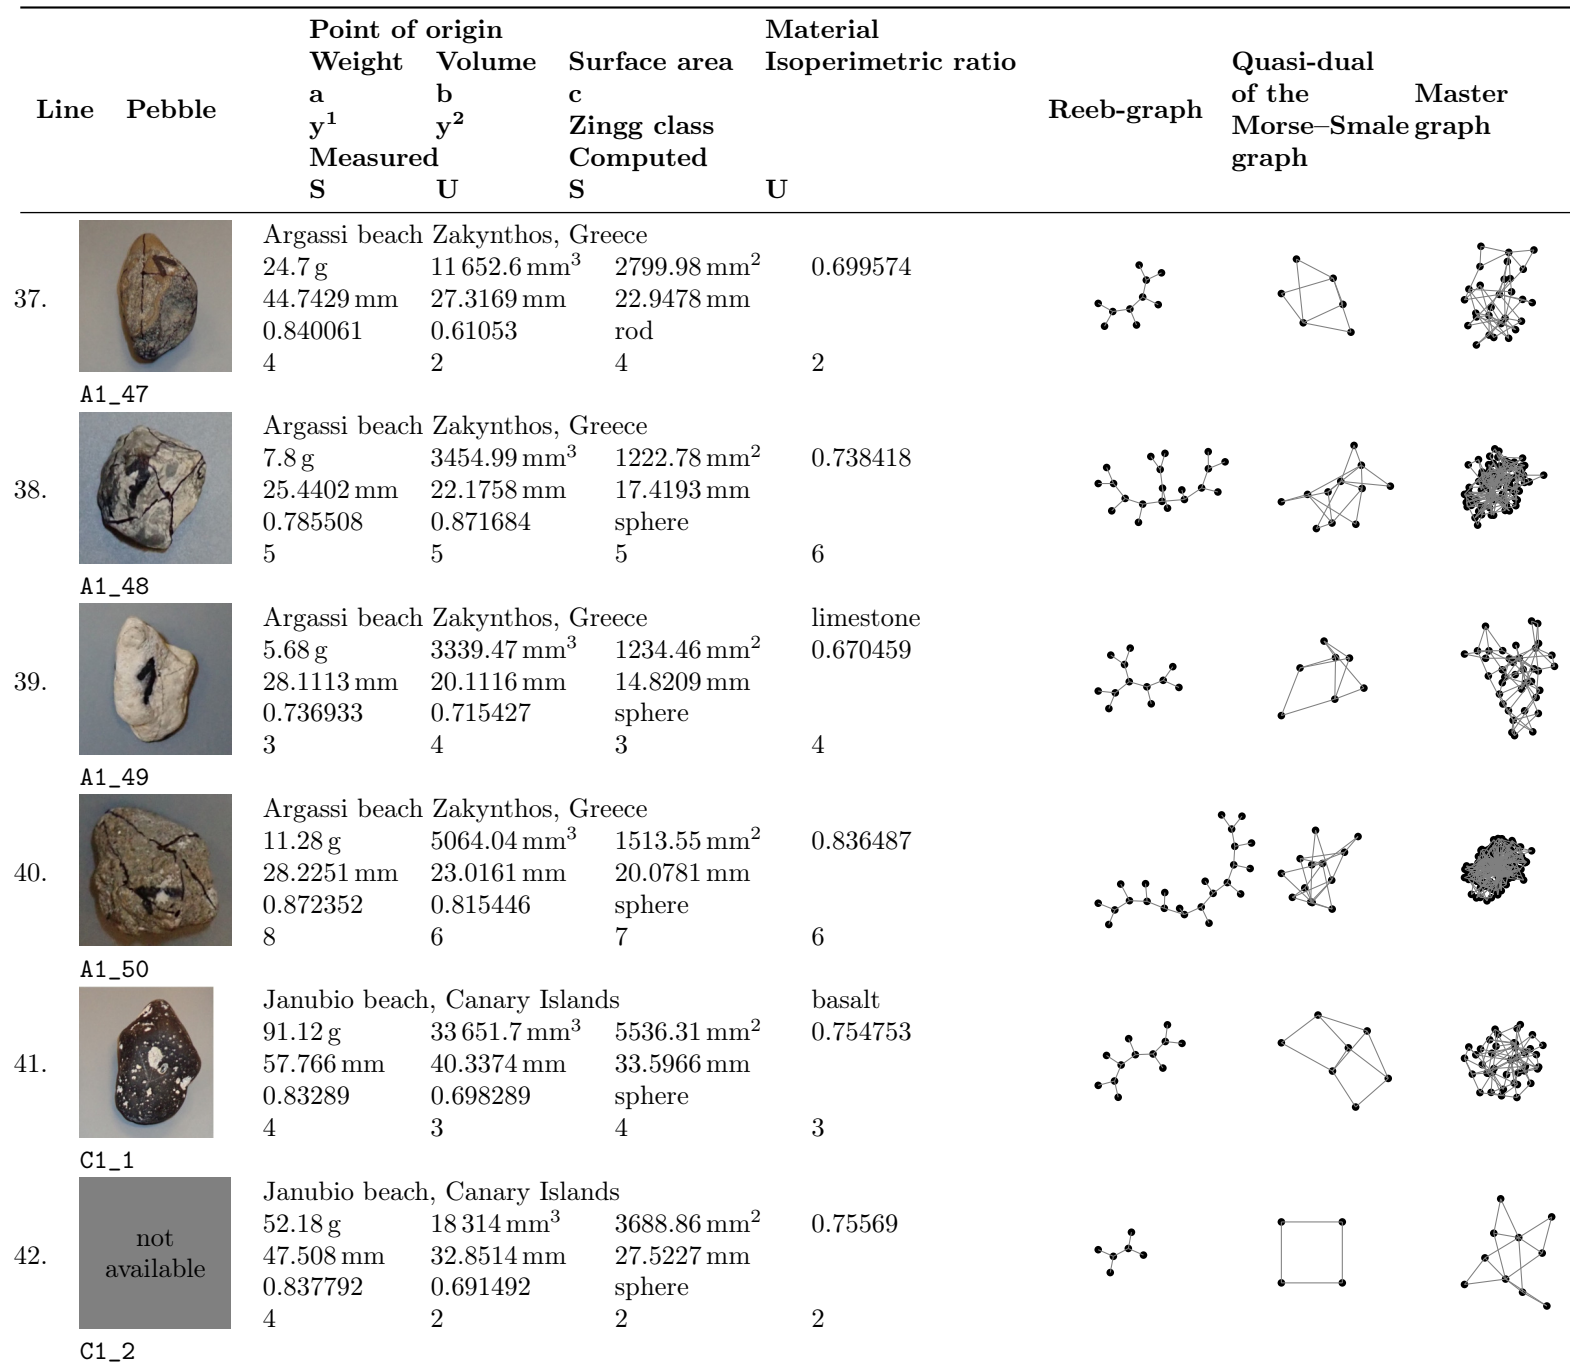 |
|      |                                                                                     | 91.12 g                              | 33 651.7 mm <sup>3</sup> |                                                      |                                      |                                                                                       |                                                                                       |                                                                                       |
|      |                                                                                     | 57.766 mm                            | 40.3374 mm               |                                                      |                                      |                                                                                       |                                                                                       |                                                                                       |
|      |                                                                                     | 0.83289                              | 0.698289                 |                                                      |                                      |                                                                                       |                                                                                       |                                                                                       |
|      | C1_1                                                                                | 4                                    | 3                        |                                                      |                                      |                                                                                       |                                                                                       |                                                                                       |
| 42.  | 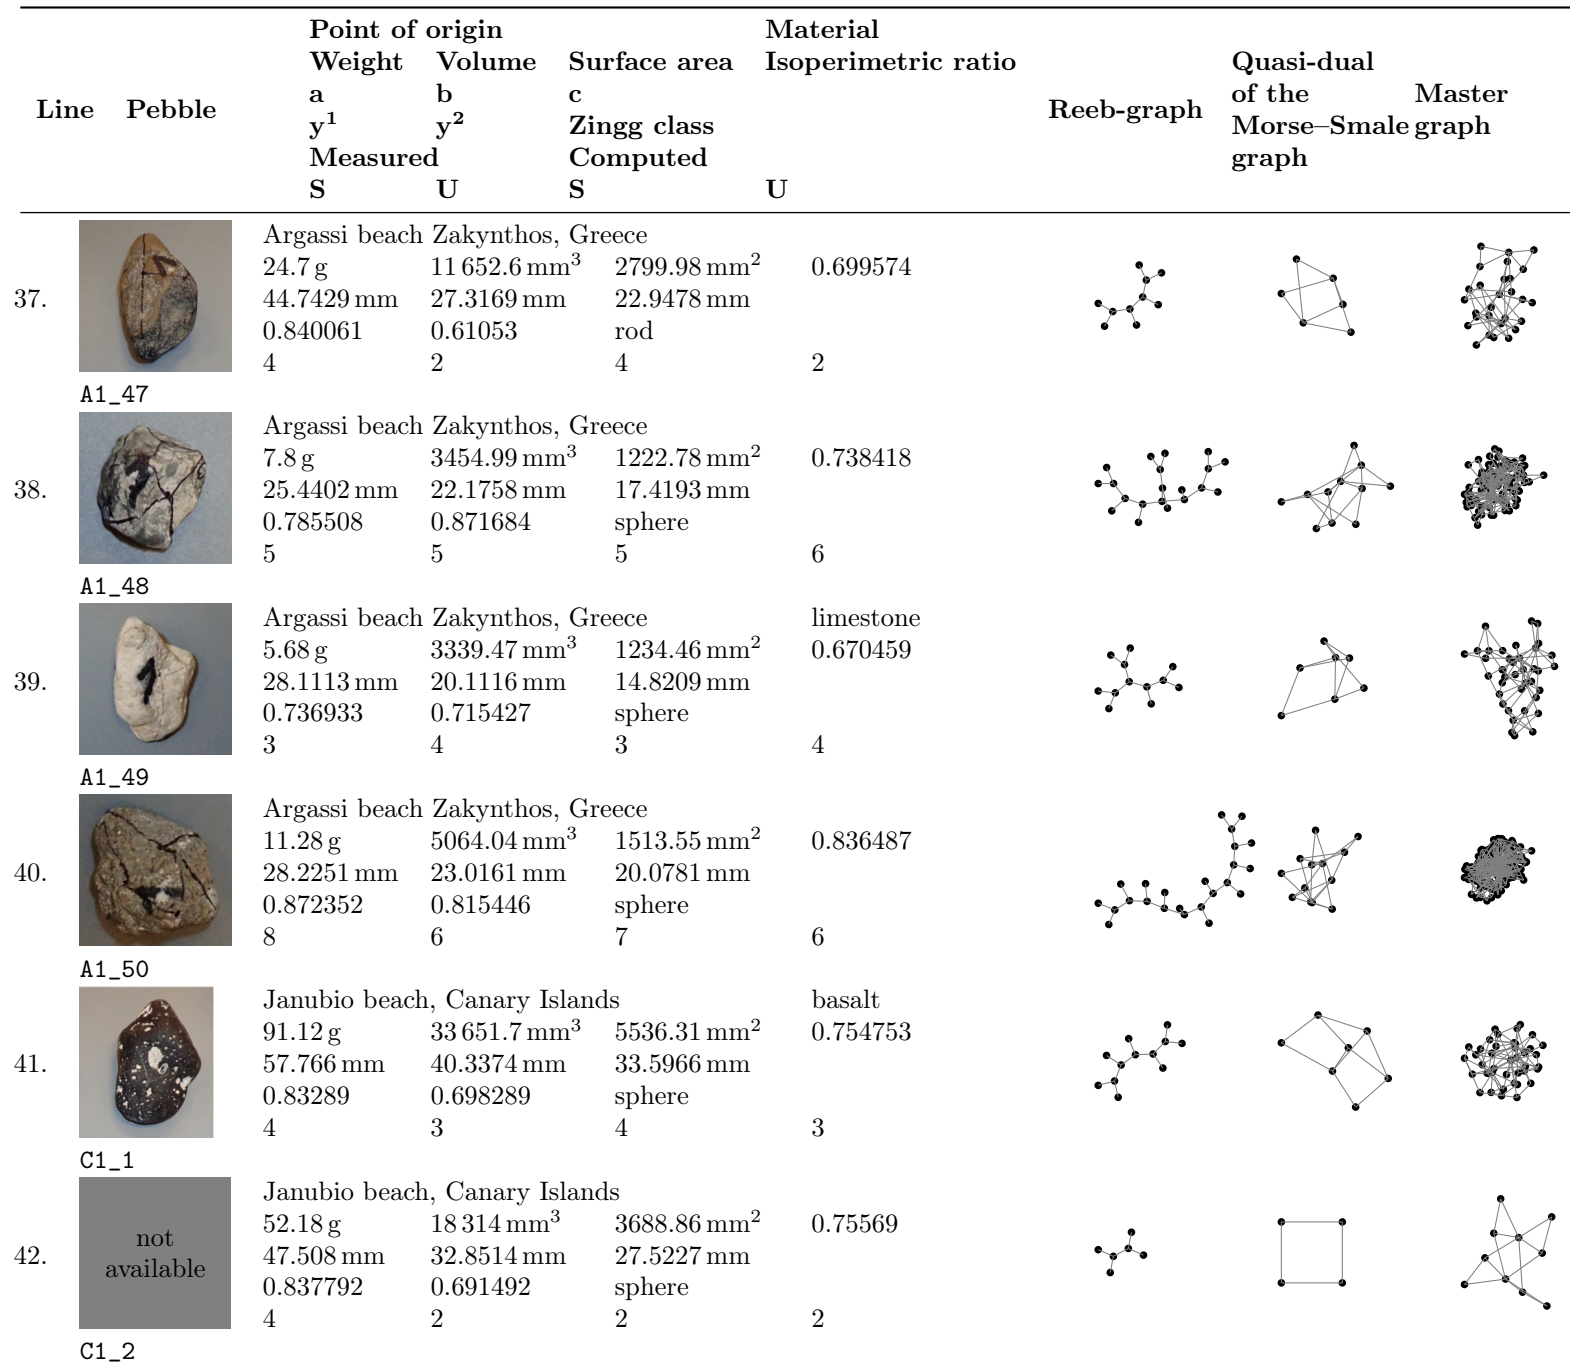 | Janubio beach, Canary Islands        |                          | 3688.86 mm <sup>2</sup><br>27.5227 mm<br>sphere<br>2 | 0.75569<br>2                         | 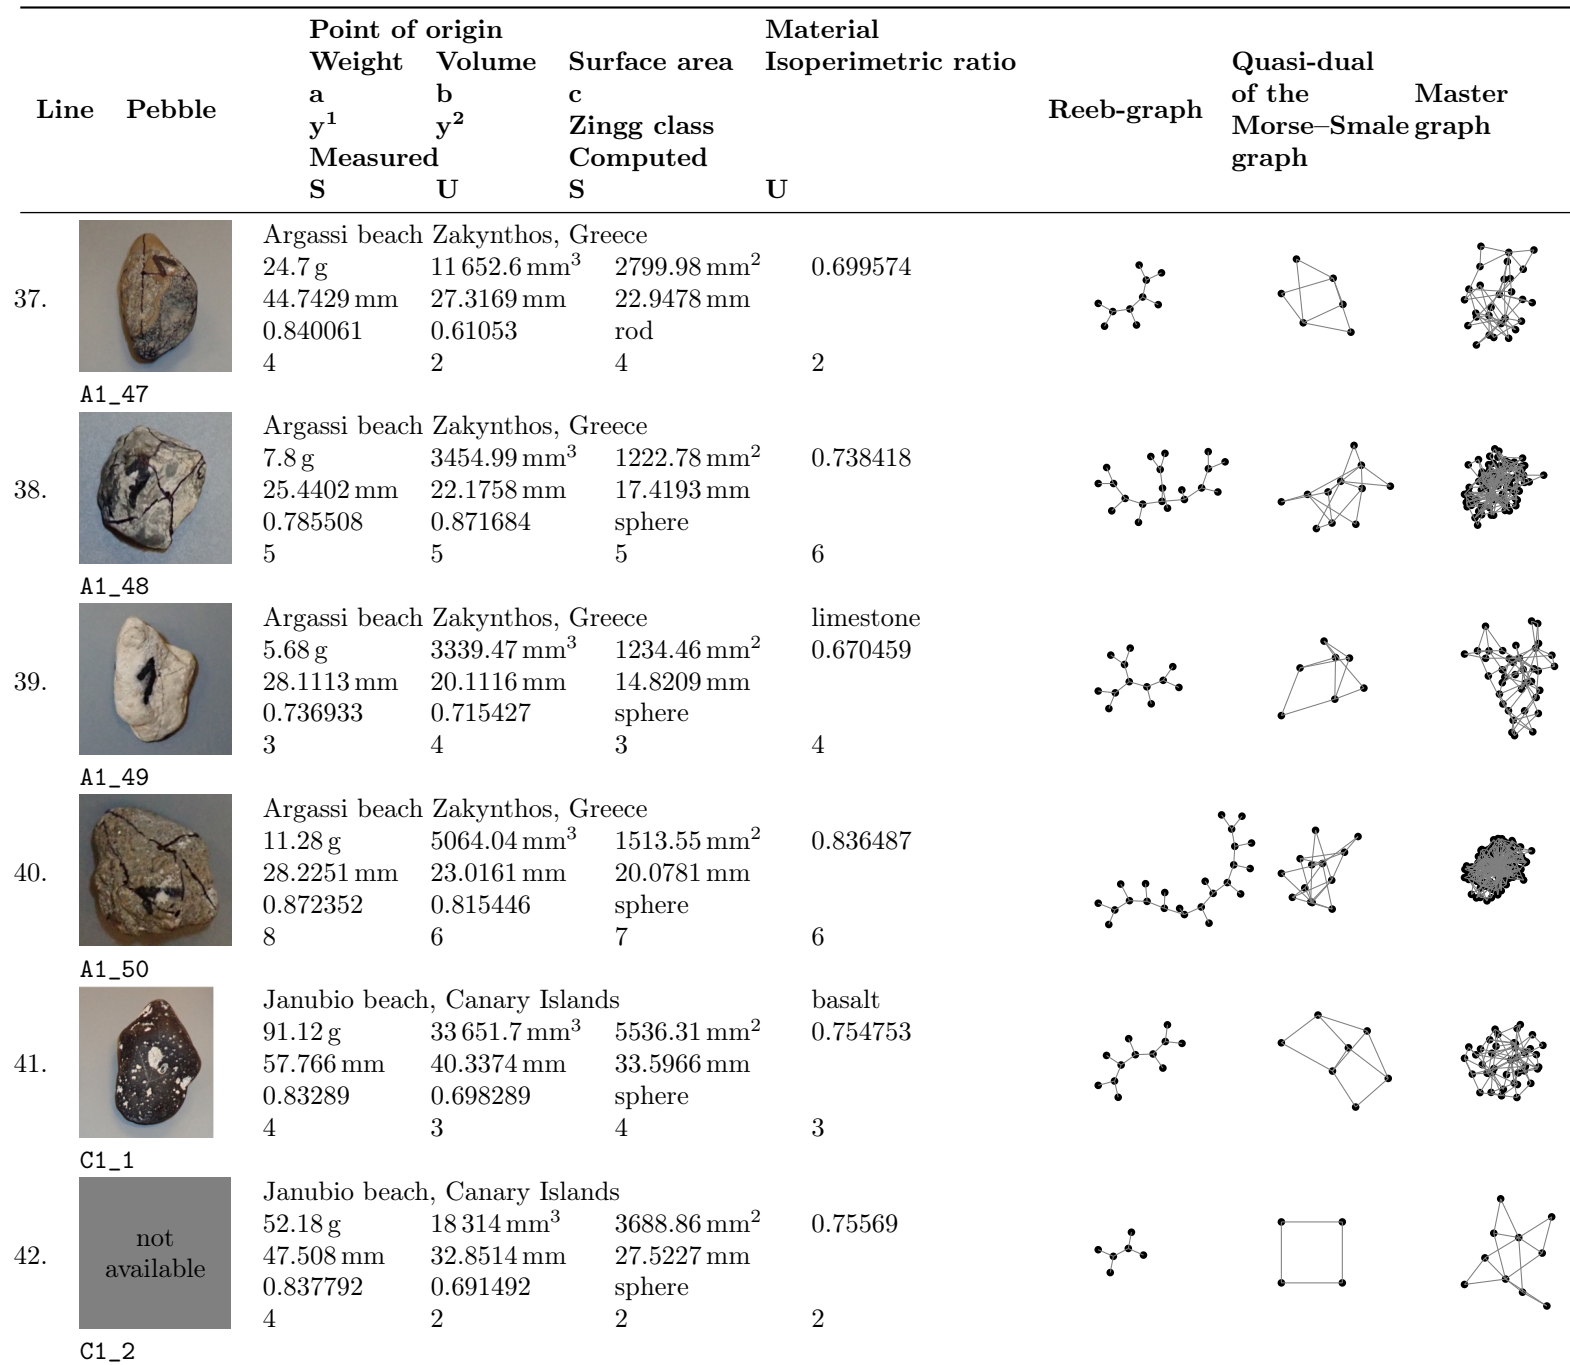 | 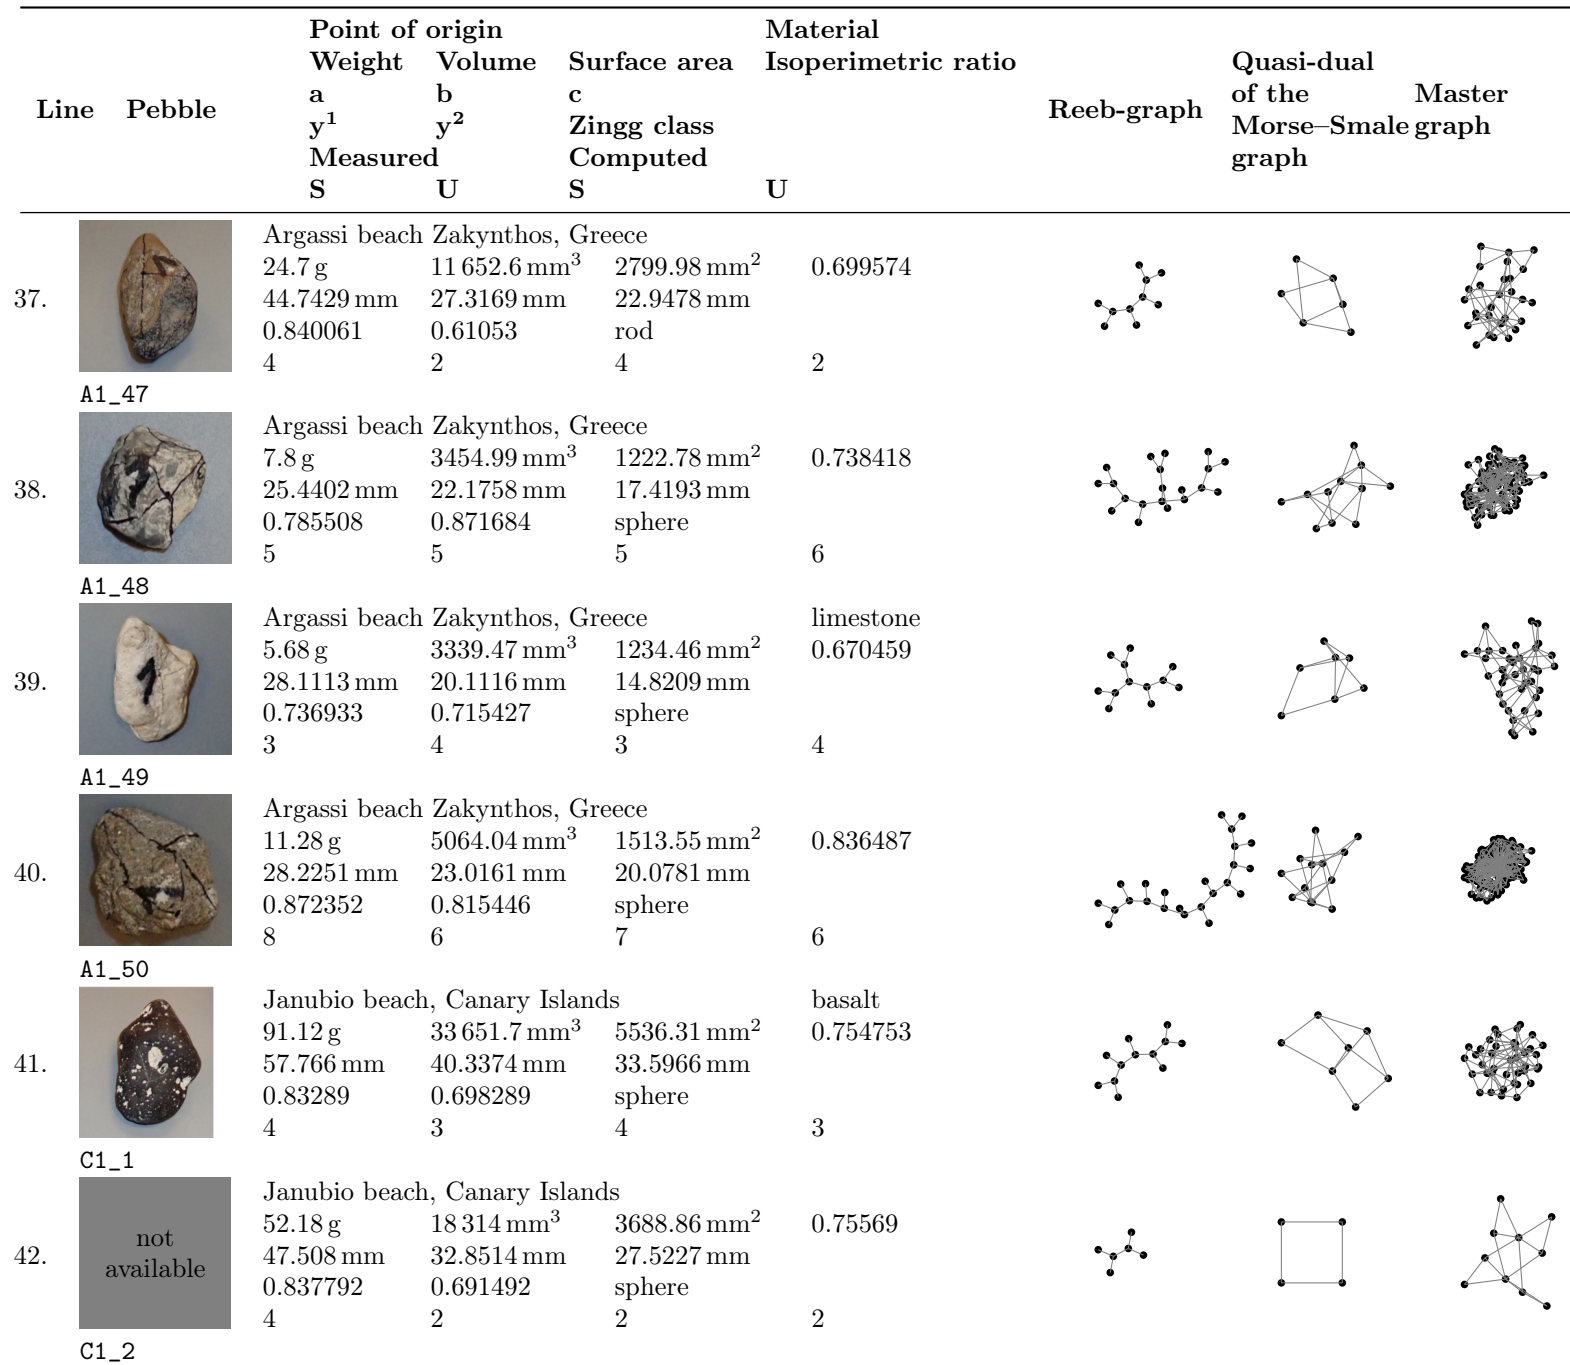 | 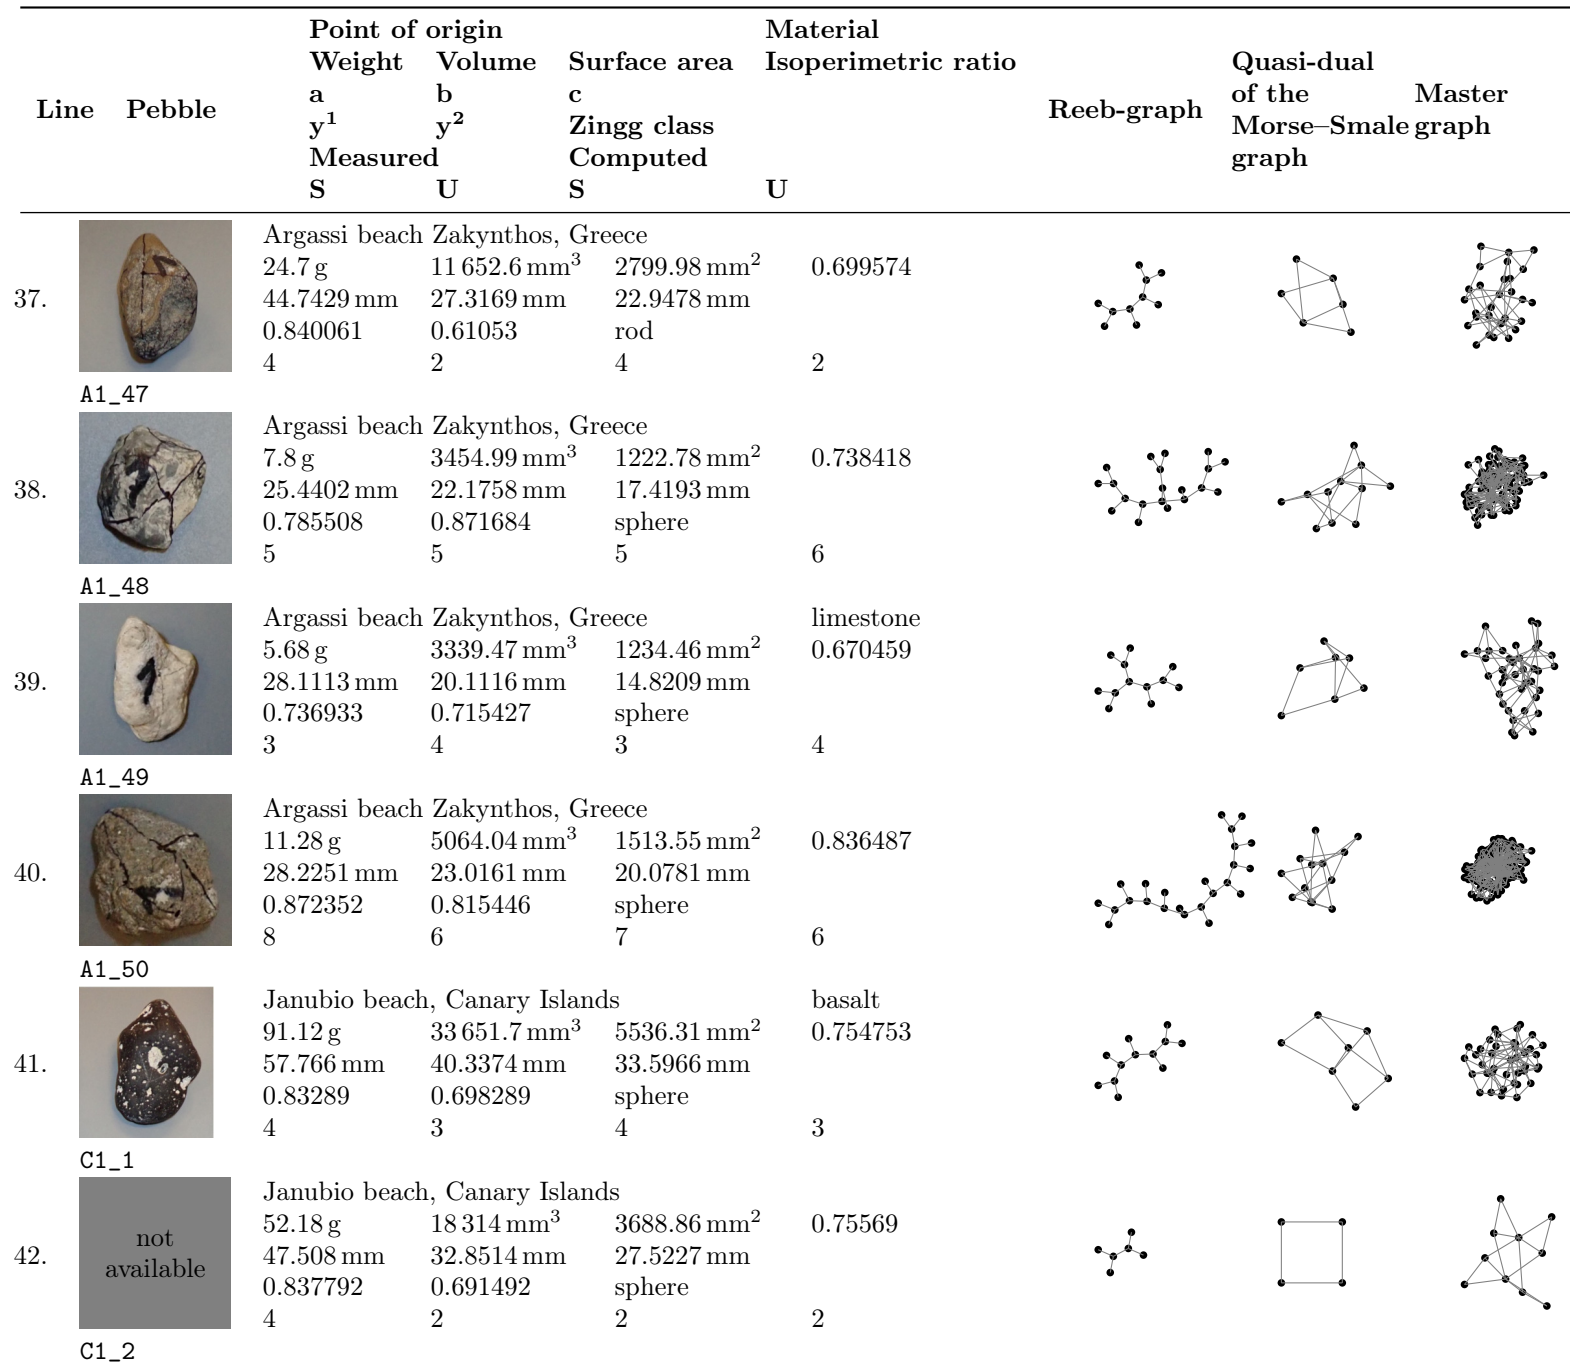 |
|      |                                                                                     | 52.18 g                              | 18 314 mm <sup>3</sup>   |                                                      |                                      |                                                                                       |                                                                                       |                                                                                       |
|      |                                                                                     | 47.508 mm                            | 32.8514 mm               |                                                      |                                      |                                                                                       |                                                                                       |                                                                                       |
|      |                                                                                     | 0.837792                             | 0.691492                 |                                                      |                                      |                                                                                       |                                                                                       |                                                                                       |
|      | C1_2                                                                                | 4                                    | 2                        |                                                      |                                      |                                                                                       |                                                                                       |                                                                                       |

| Line | Pebble                                                                              | Point of origin               |                          |                         | Material | Isoperimetric ratio | Reeb-graph                                                                            | Quasi-dual<br>of the<br>Morse–Smale<br>graph                                          | Master<br>graph                                                                       |
|------|-------------------------------------------------------------------------------------|-------------------------------|--------------------------|-------------------------|----------|---------------------|---------------------------------------------------------------------------------------|---------------------------------------------------------------------------------------|---------------------------------------------------------------------------------------|
|      |                                                                                     | Weight                        | Volume                   | Surface area            |          |                     |                                                                                       |                                                                                       |                                                                                       |
|      |                                                                                     | a                             | b                        | c                       |          |                     |                                                                                       |                                                                                       |                                                                                       |
|      |                                                                                     | y <sup>1</sup>                | y <sup>2</sup>           | Zingg class             |          |                     |                                                                                       |                                                                                       |                                                                                       |
|      |                                                                                     | Measured                      | U                        | Computed                | U        |                     |                                                                                       |                                                                                       |                                                                                       |
| S    | S                                                                                   | S                             | S                        | S                       | U        |                     |                                                                                       |                                                                                       |                                                                                       |
| 43.  | 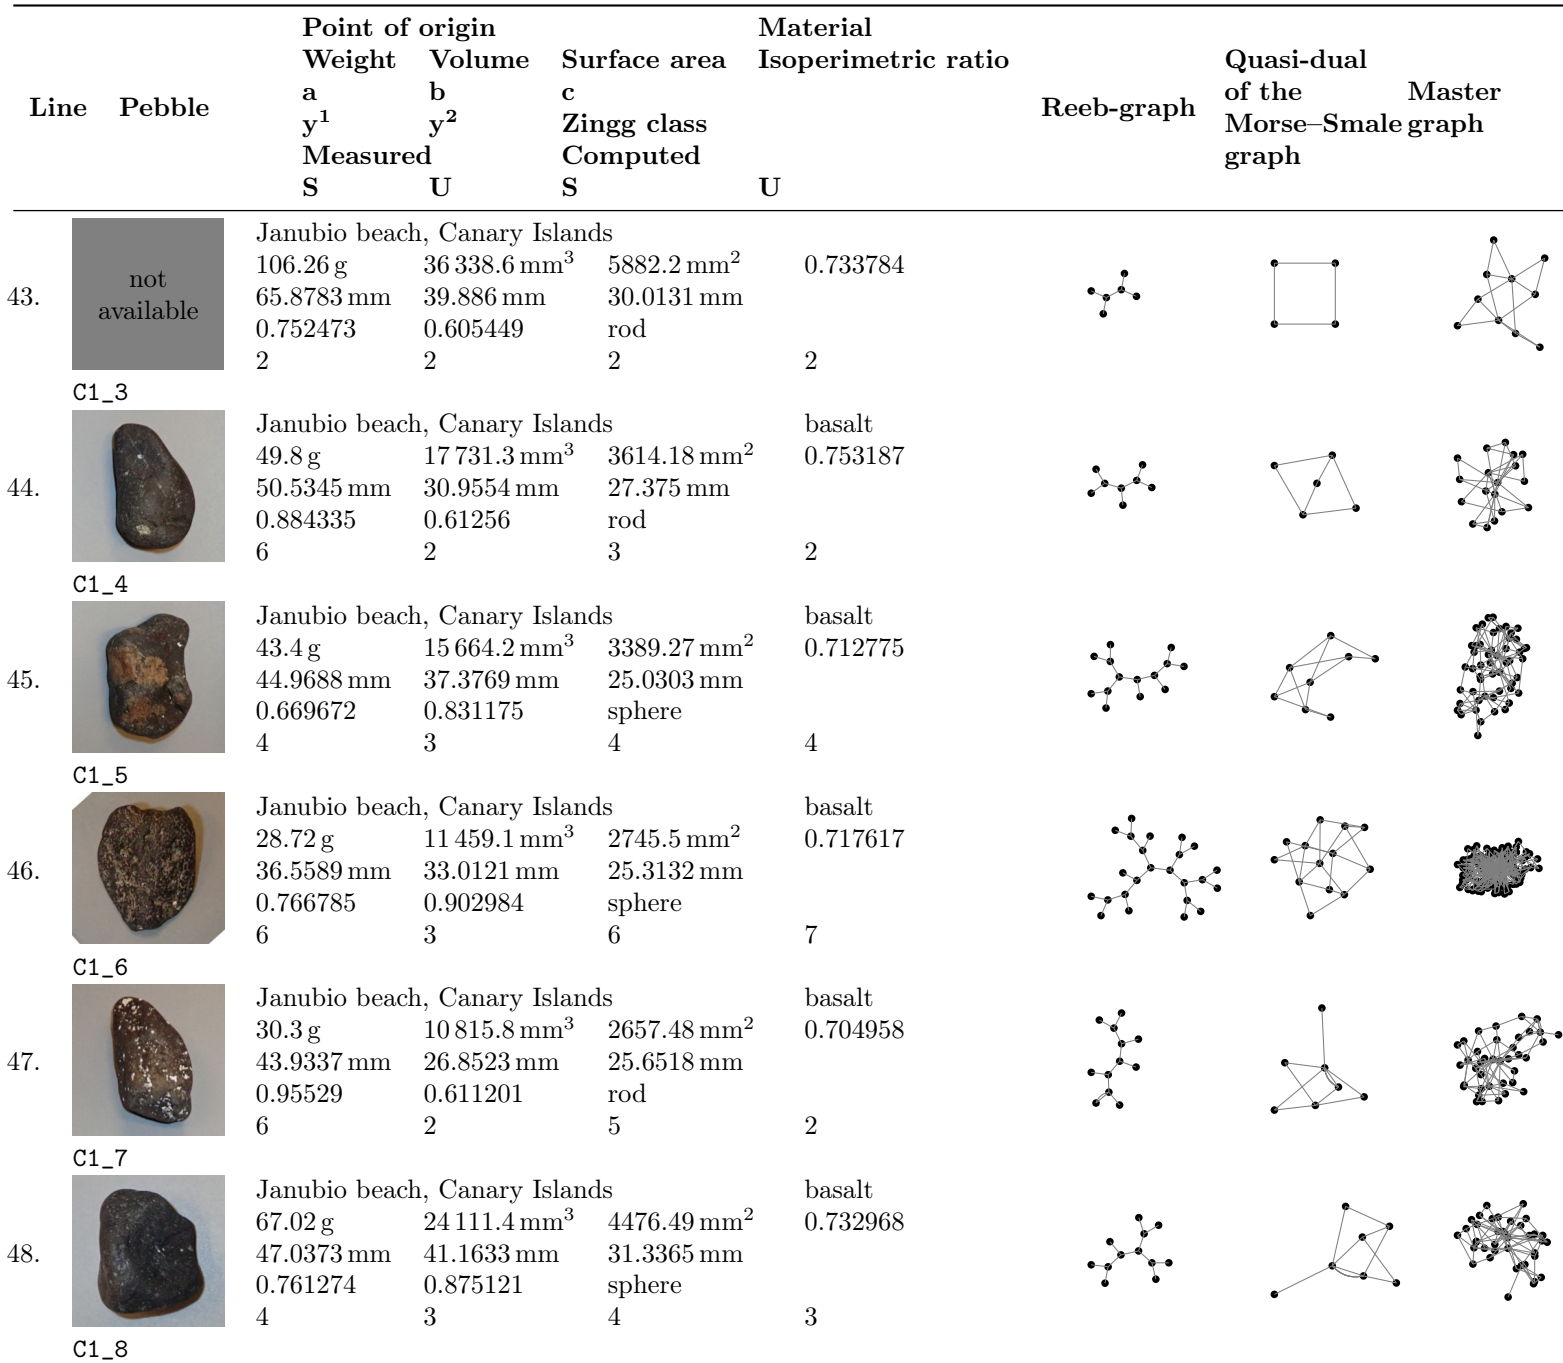   | Janubio beach, Canary Islands |                          |                         |          | 0.733784            | 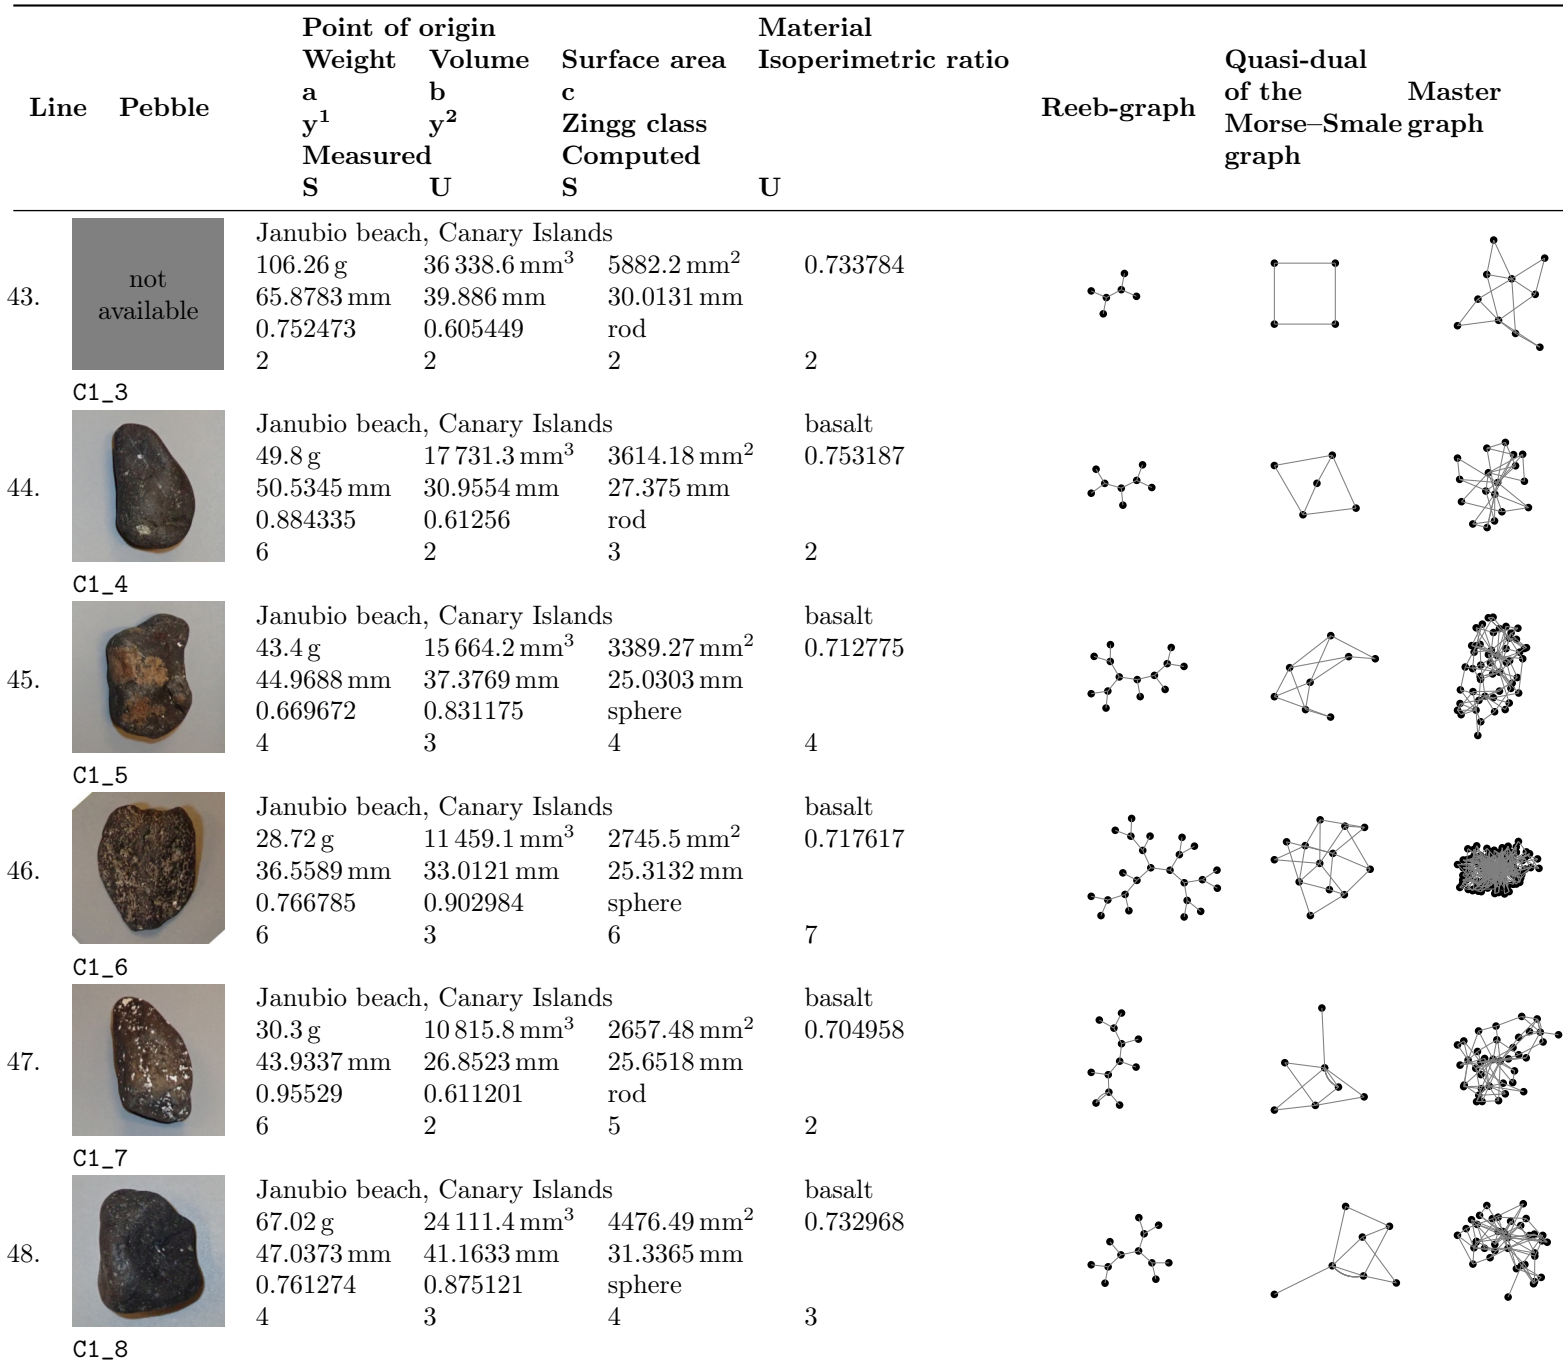   | 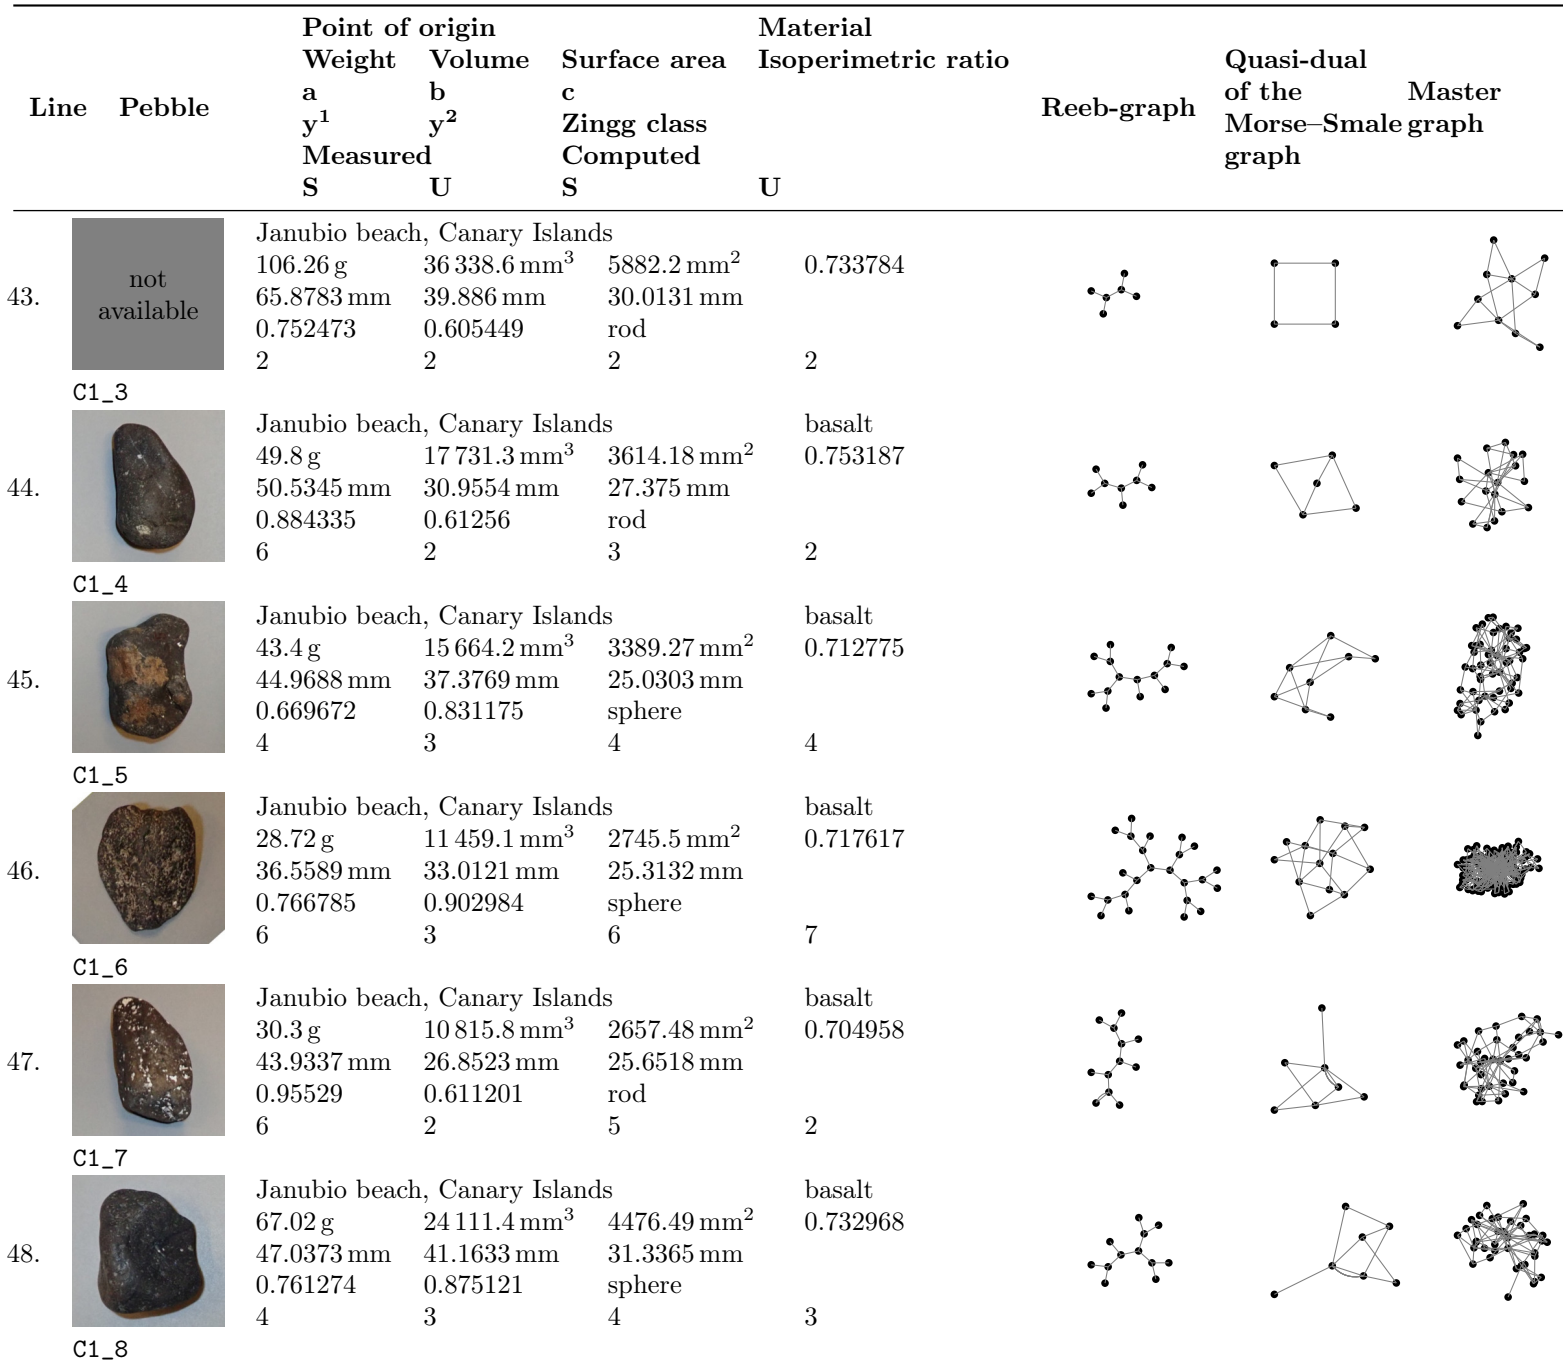   | 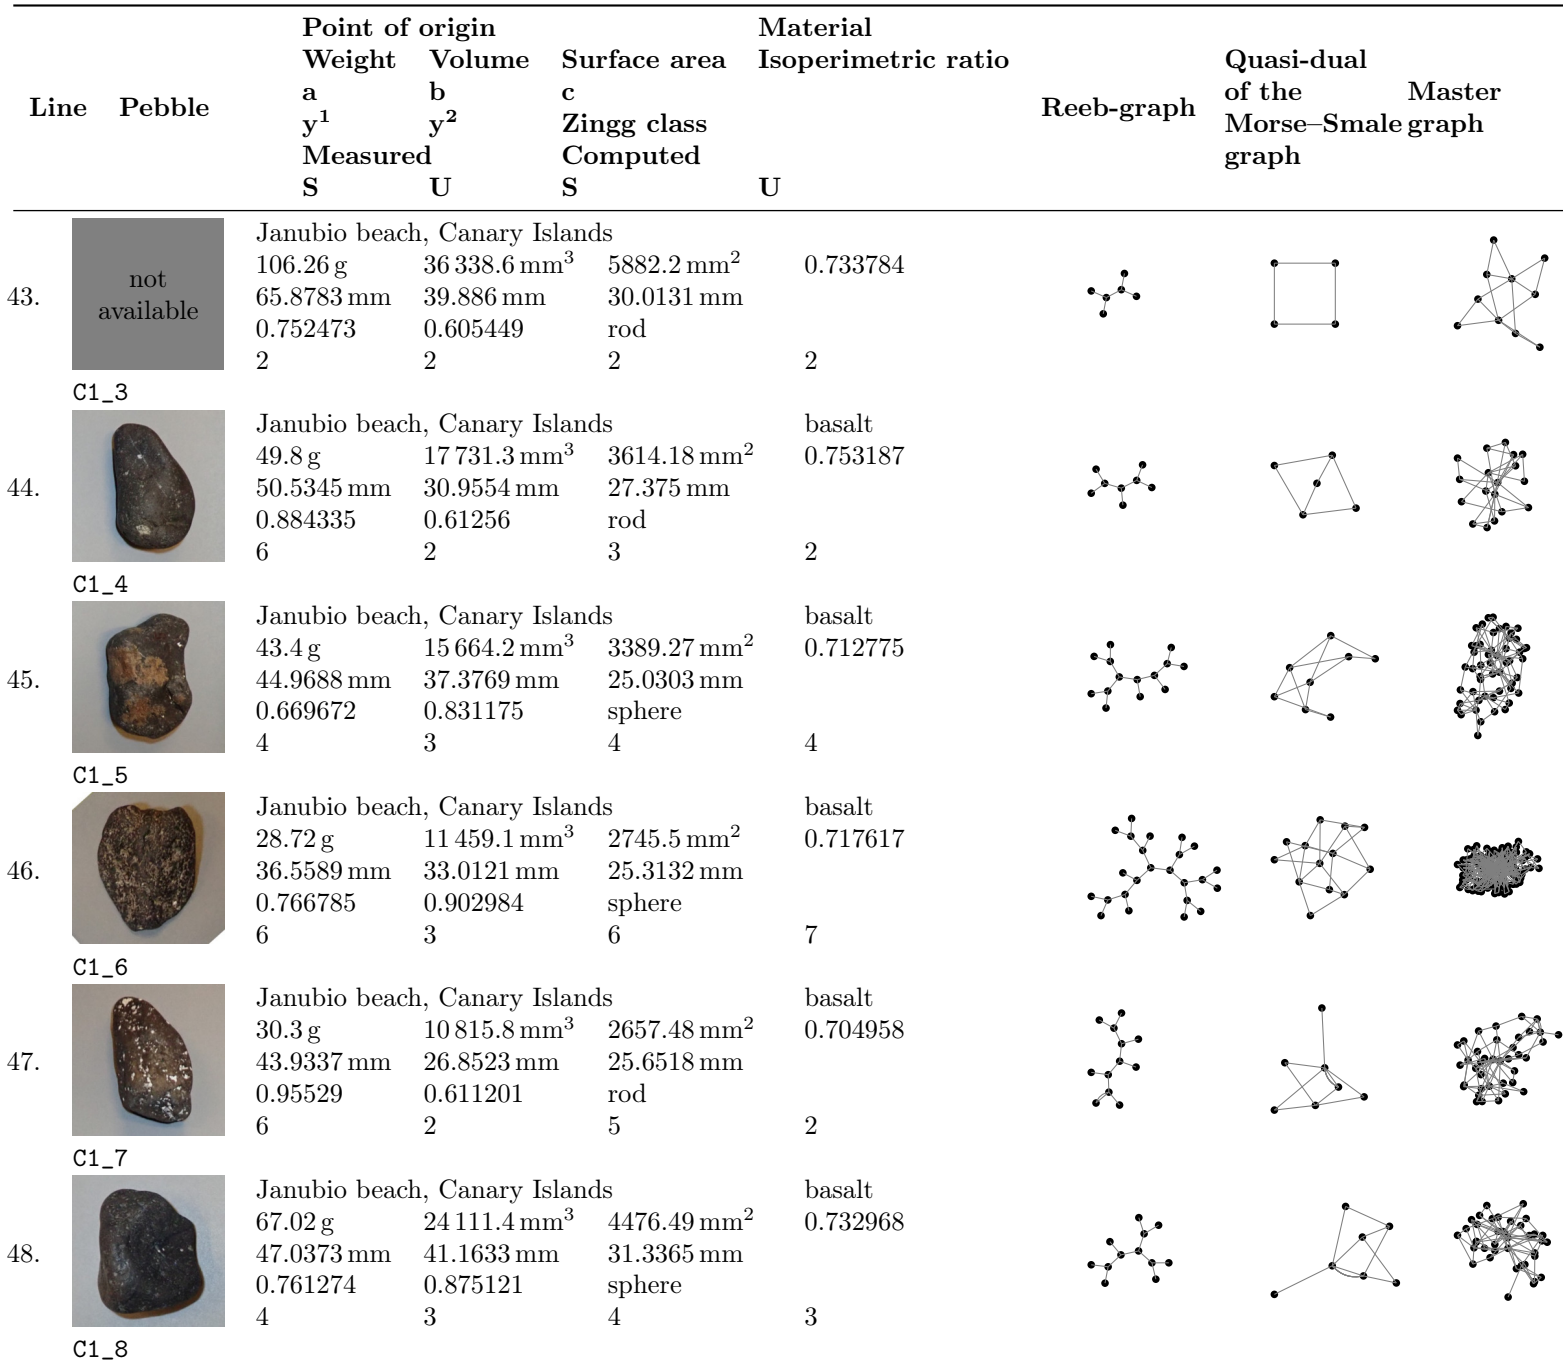   |
|      |                                                                                     | 106.26 g                      | 36 338.6 mm <sup>3</sup> | 5882.2 mm <sup>2</sup>  |          |                     |                                                                                       |                                                                                       |                                                                                       |
|      |                                                                                     | 65.8783 mm                    | 39.886 mm                | 30.0131 mm              |          |                     |                                                                                       |                                                                                       |                                                                                       |
|      |                                                                                     | 0.752473                      | 0.605449                 | rod                     |          |                     |                                                                                       |                                                                                       |                                                                                       |
|      |                                                                                     | 2                             | 2                        | 2                       | 2        |                     |                                                                                       |                                                                                       |                                                                                       |
| C1_3 |                                                                                     |                               |                          |                         |          |                     |                                                                                       |                                                                                       |                                                                                       |
| 44.  | 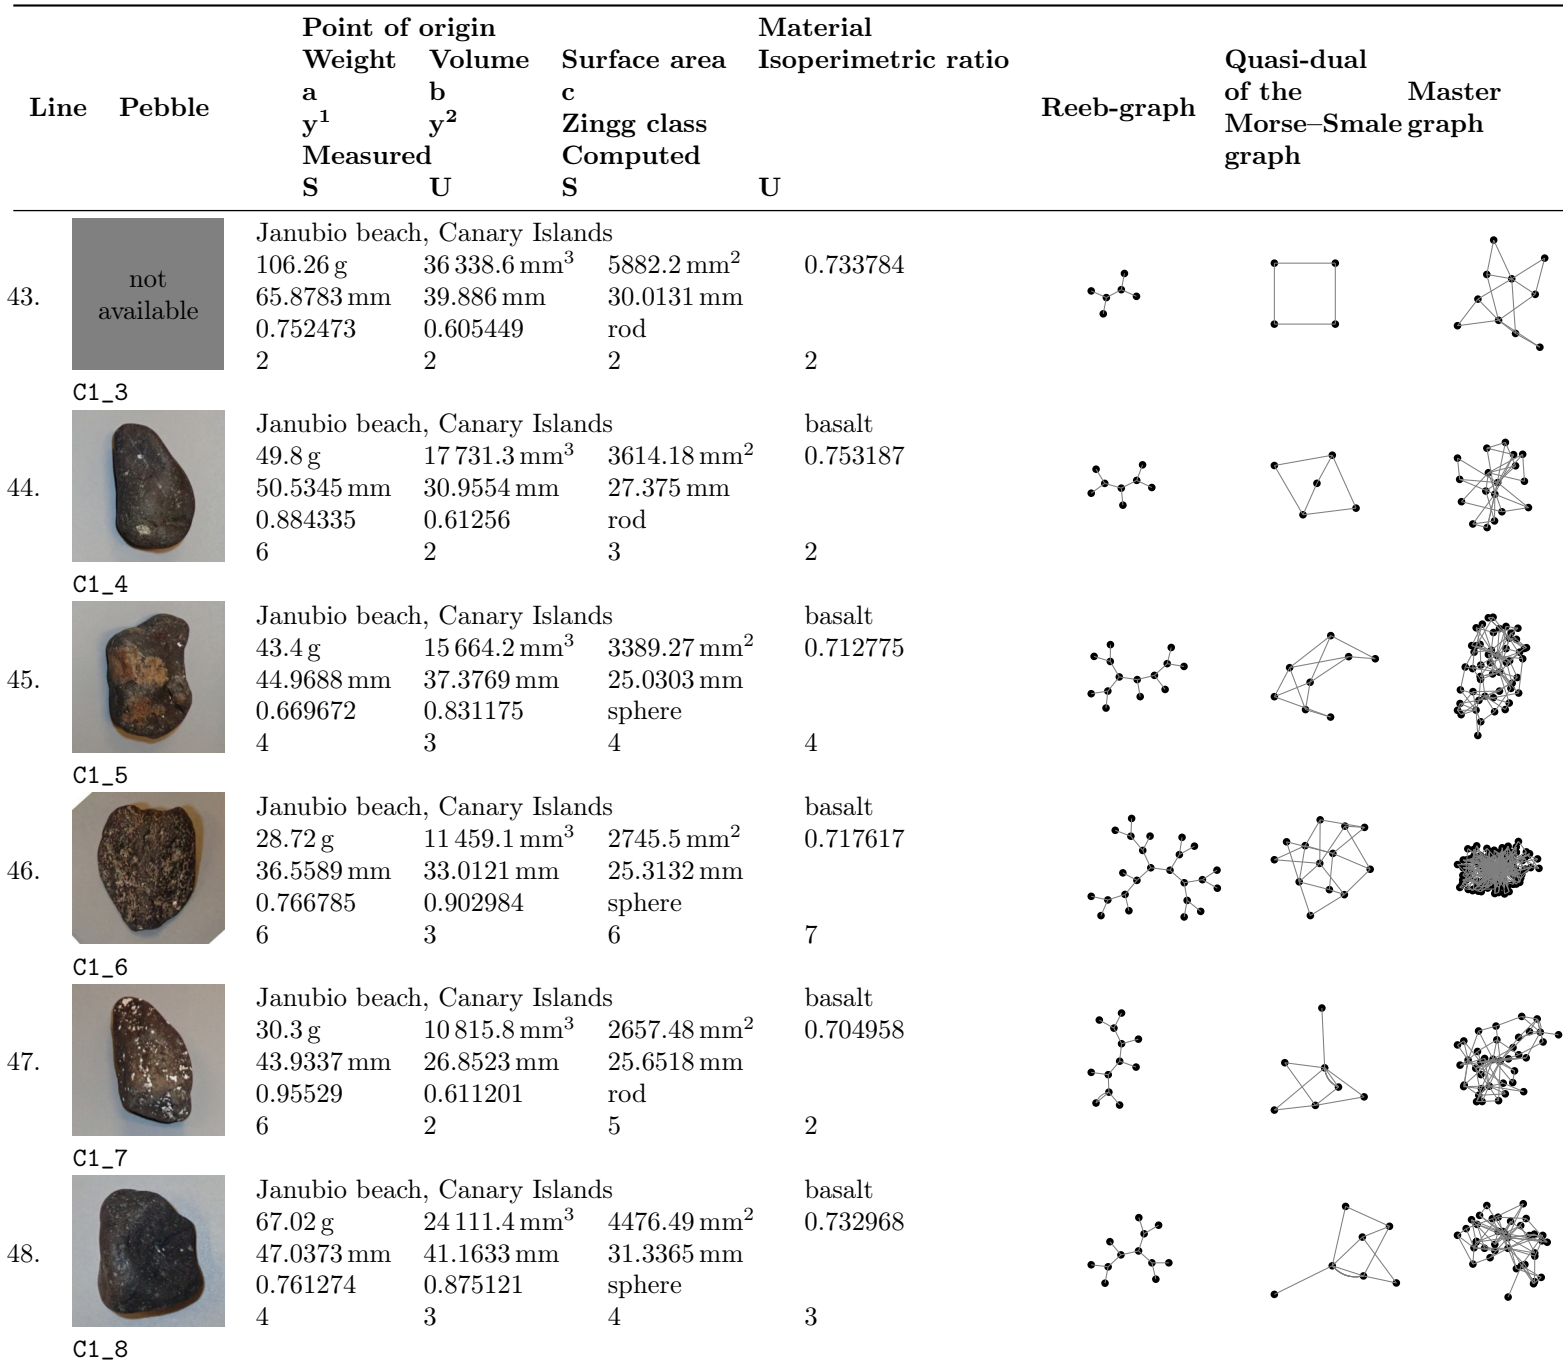   | Janubio beach, Canary Islands |                          |                         |          | basalt              | 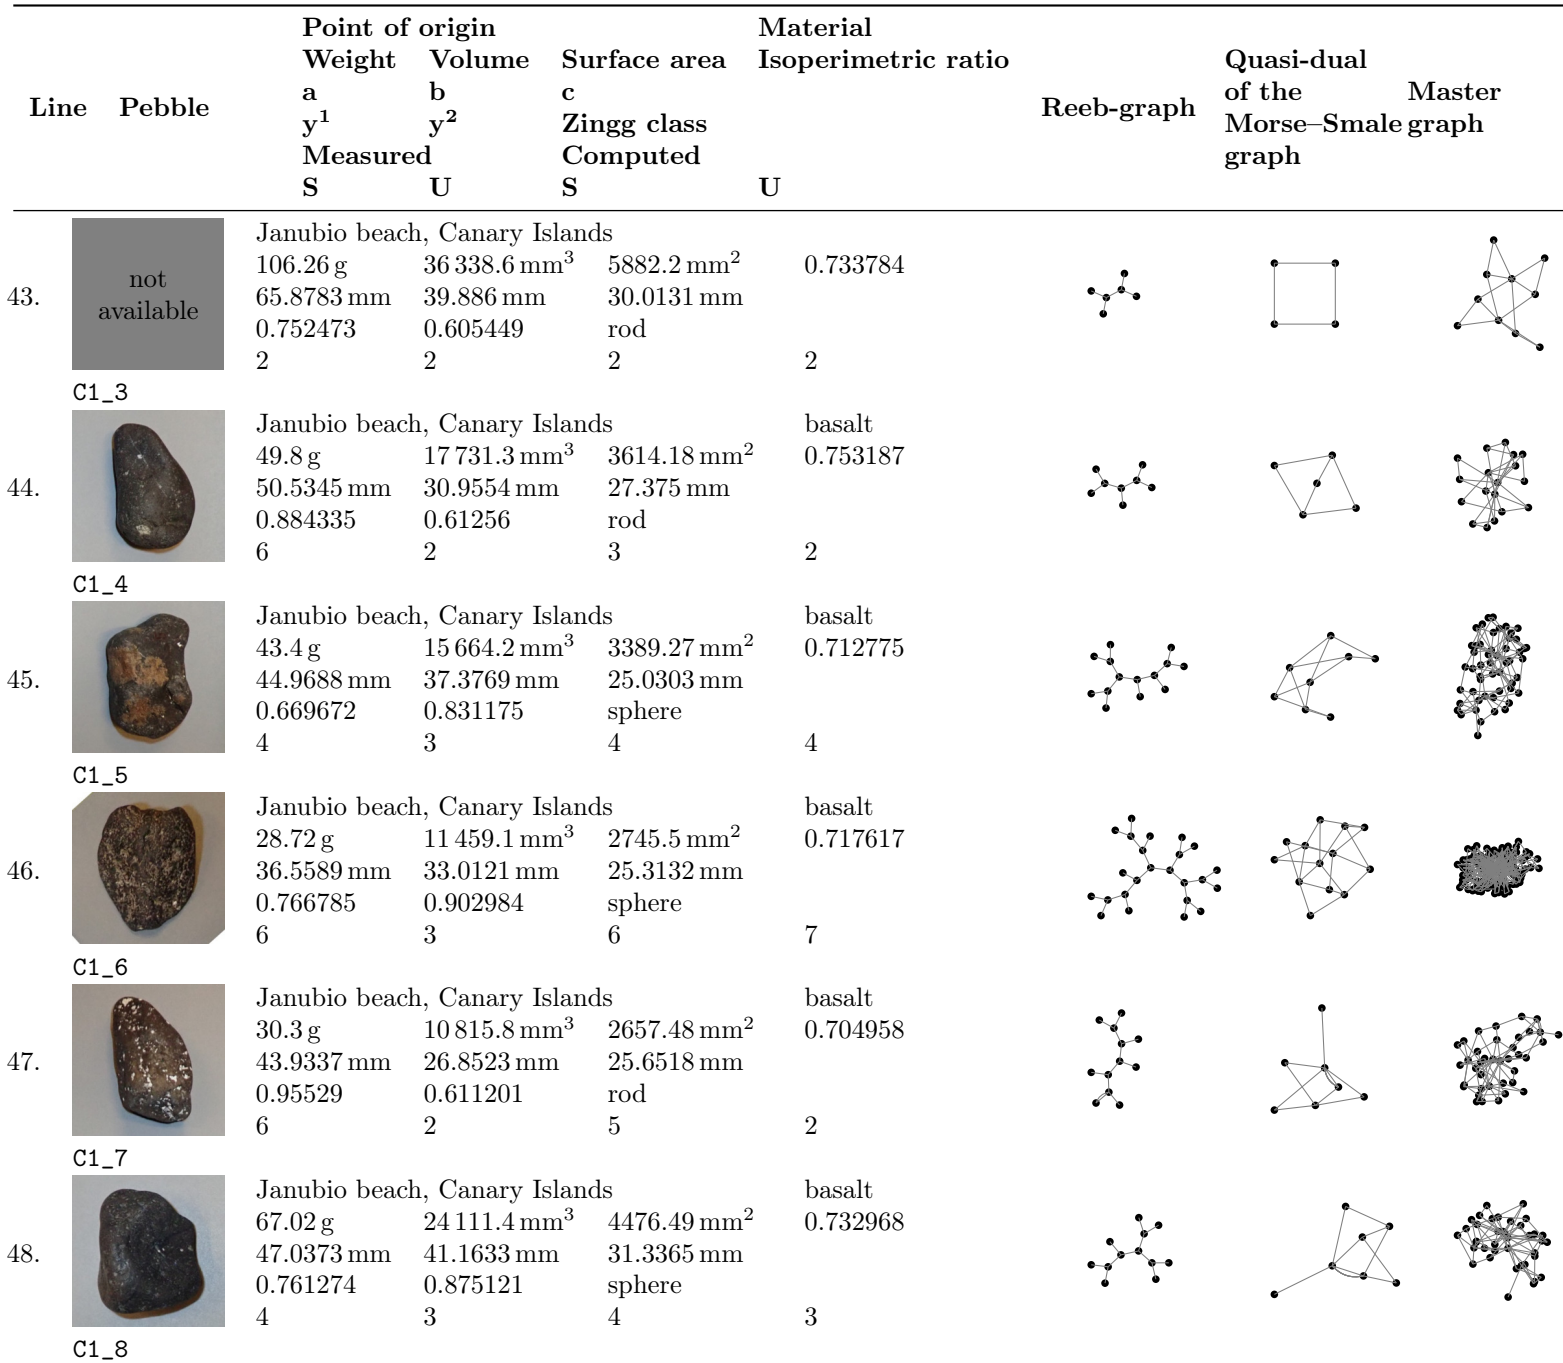   | 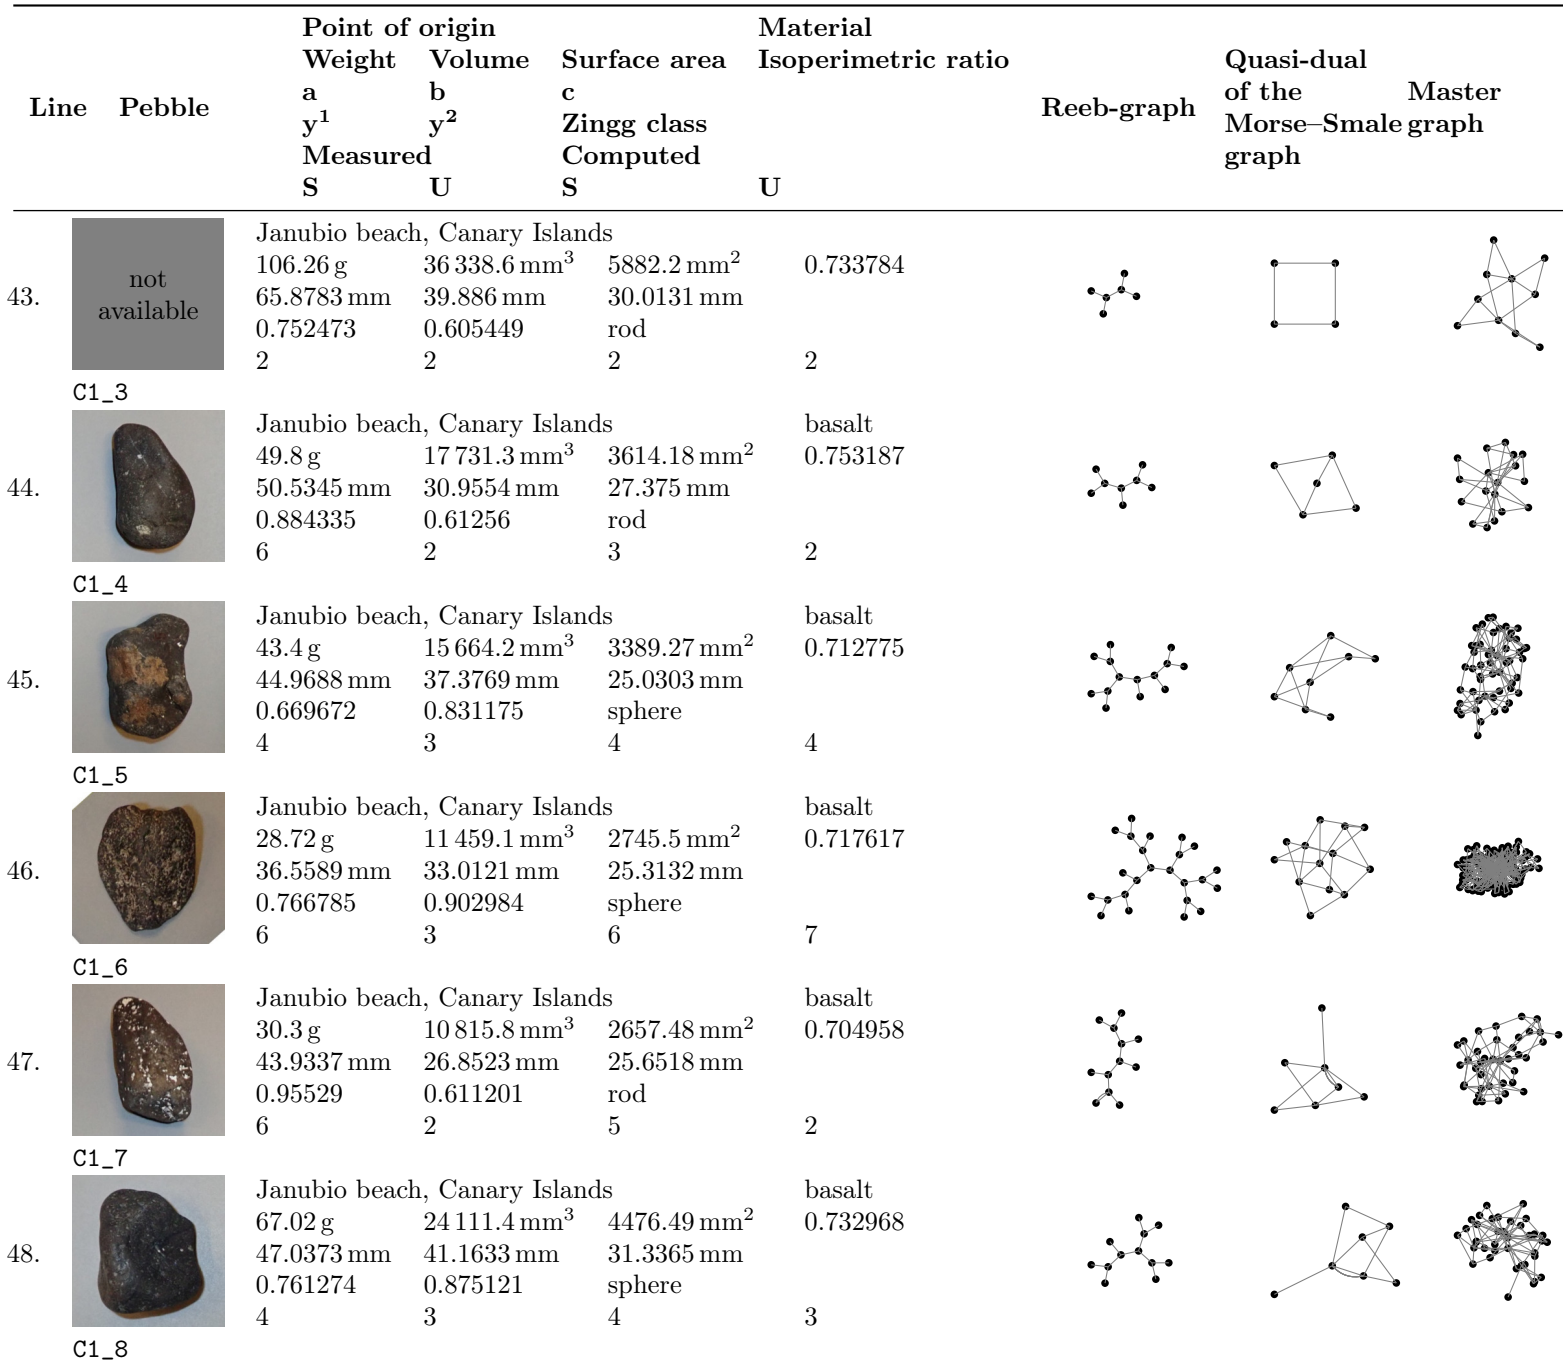   | 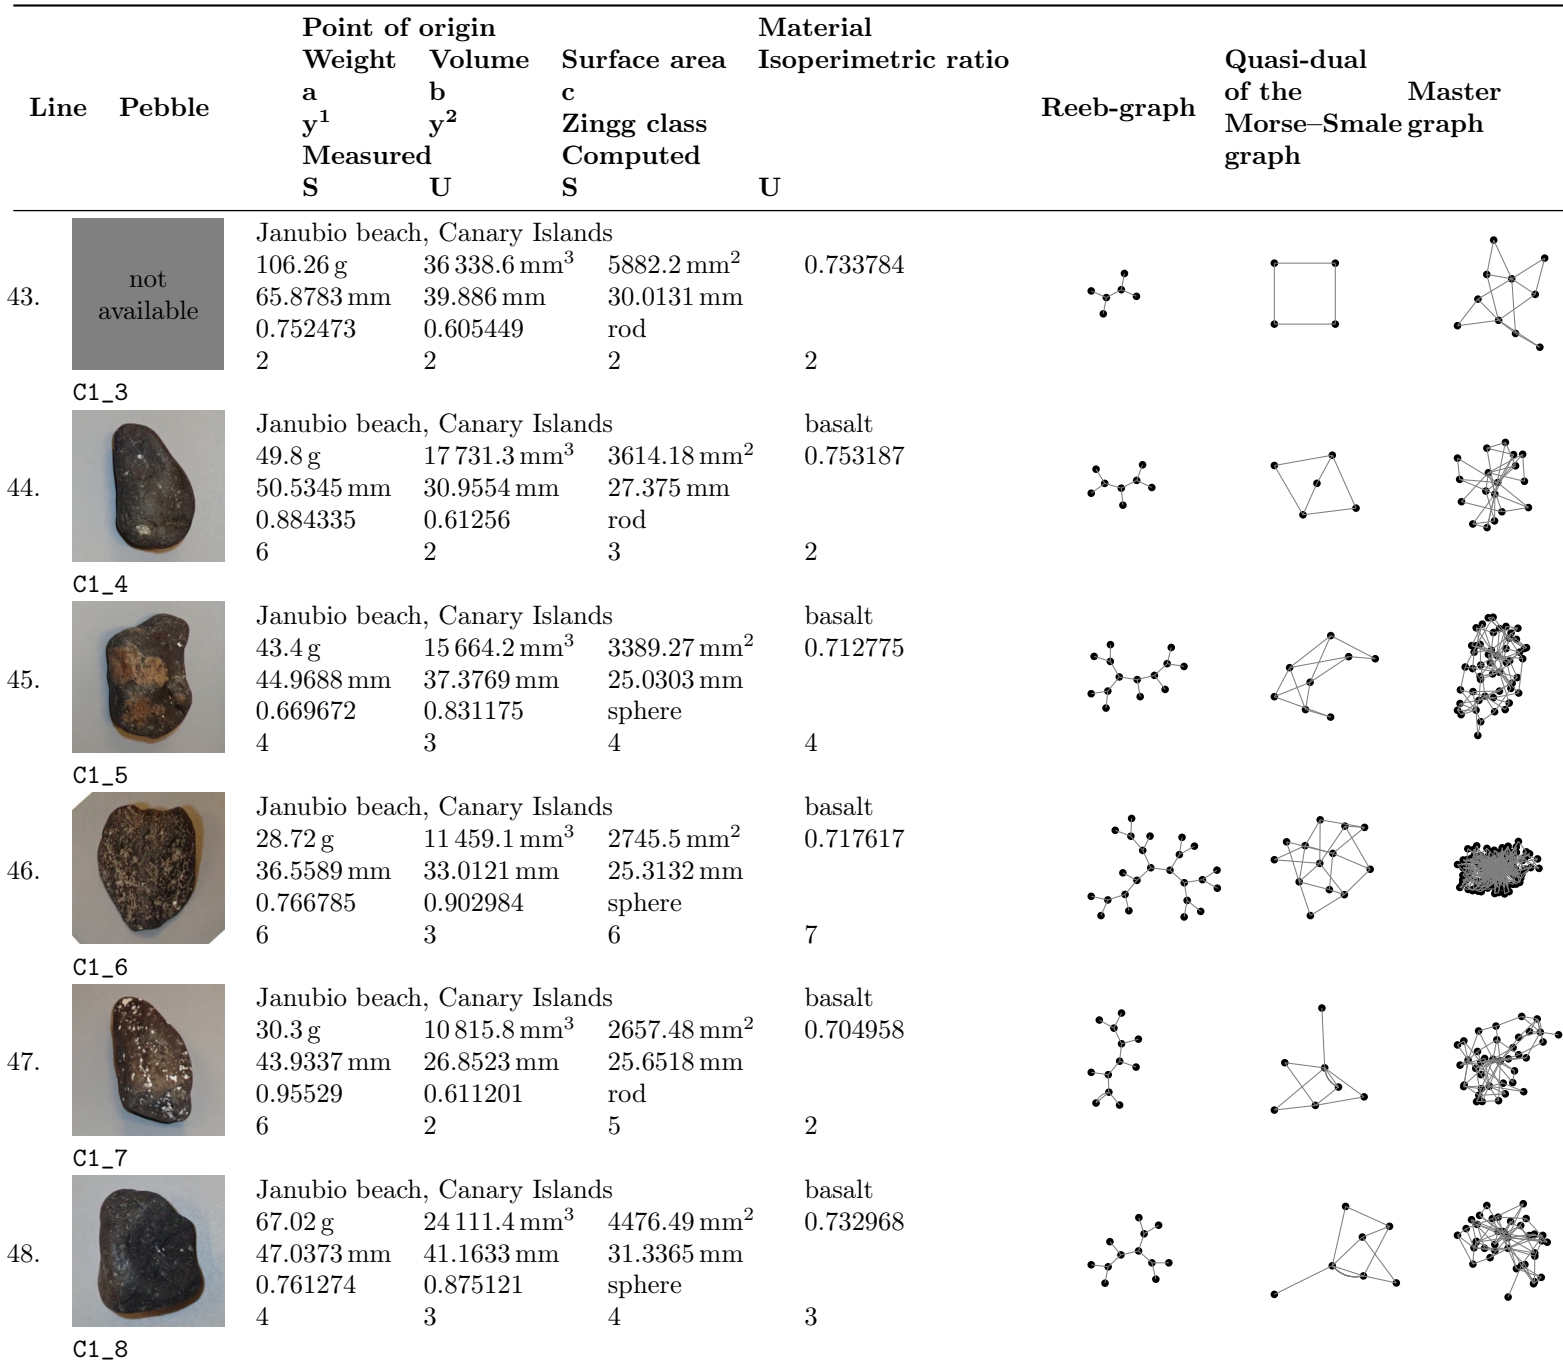   |
|      |                                                                                     | 49.8 g                        | 17 731.3 mm <sup>3</sup> | 3614.18 mm <sup>2</sup> | 0.753187 |                     |                                                                                       |                                                                                       |                                                                                       |
|      |                                                                                     | 50.5345 mm                    | 30.9554 mm               | 27.375 mm               |          |                     |                                                                                       |                                                                                       |                                                                                       |
|      |                                                                                     | 0.884335                      | 0.61256                  | rod                     |          |                     |                                                                                       |                                                                                       |                                                                                       |
|      |                                                                                     | 6                             | 2                        | 3                       | 2        |                     |                                                                                       |                                                                                       |                                                                                       |
| C1_4 |                                                                                     |                               |                          |                         |          |                     |                                                                                       |                                                                                       |                                                                                       |
| 45.  | 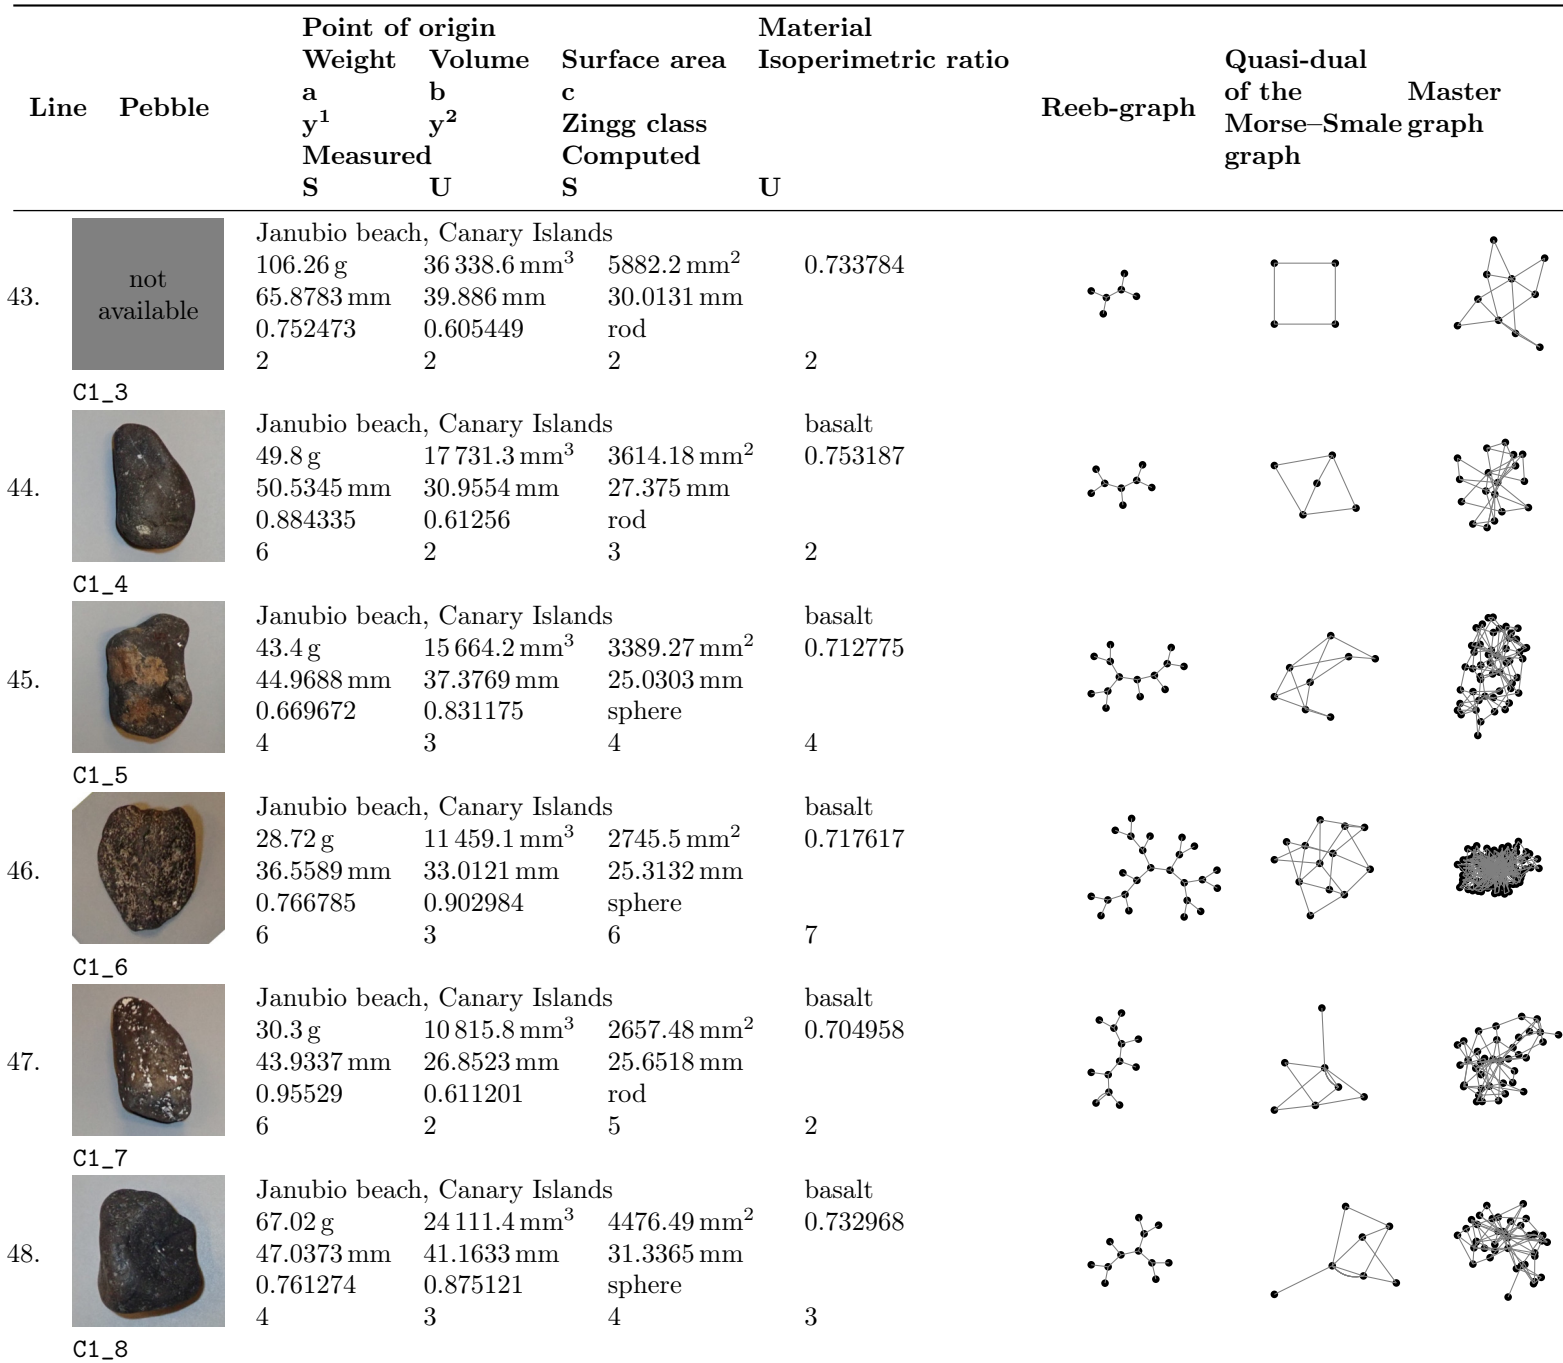   | Janubio beach, Canary Islands |                          |                         |          | basalt              | 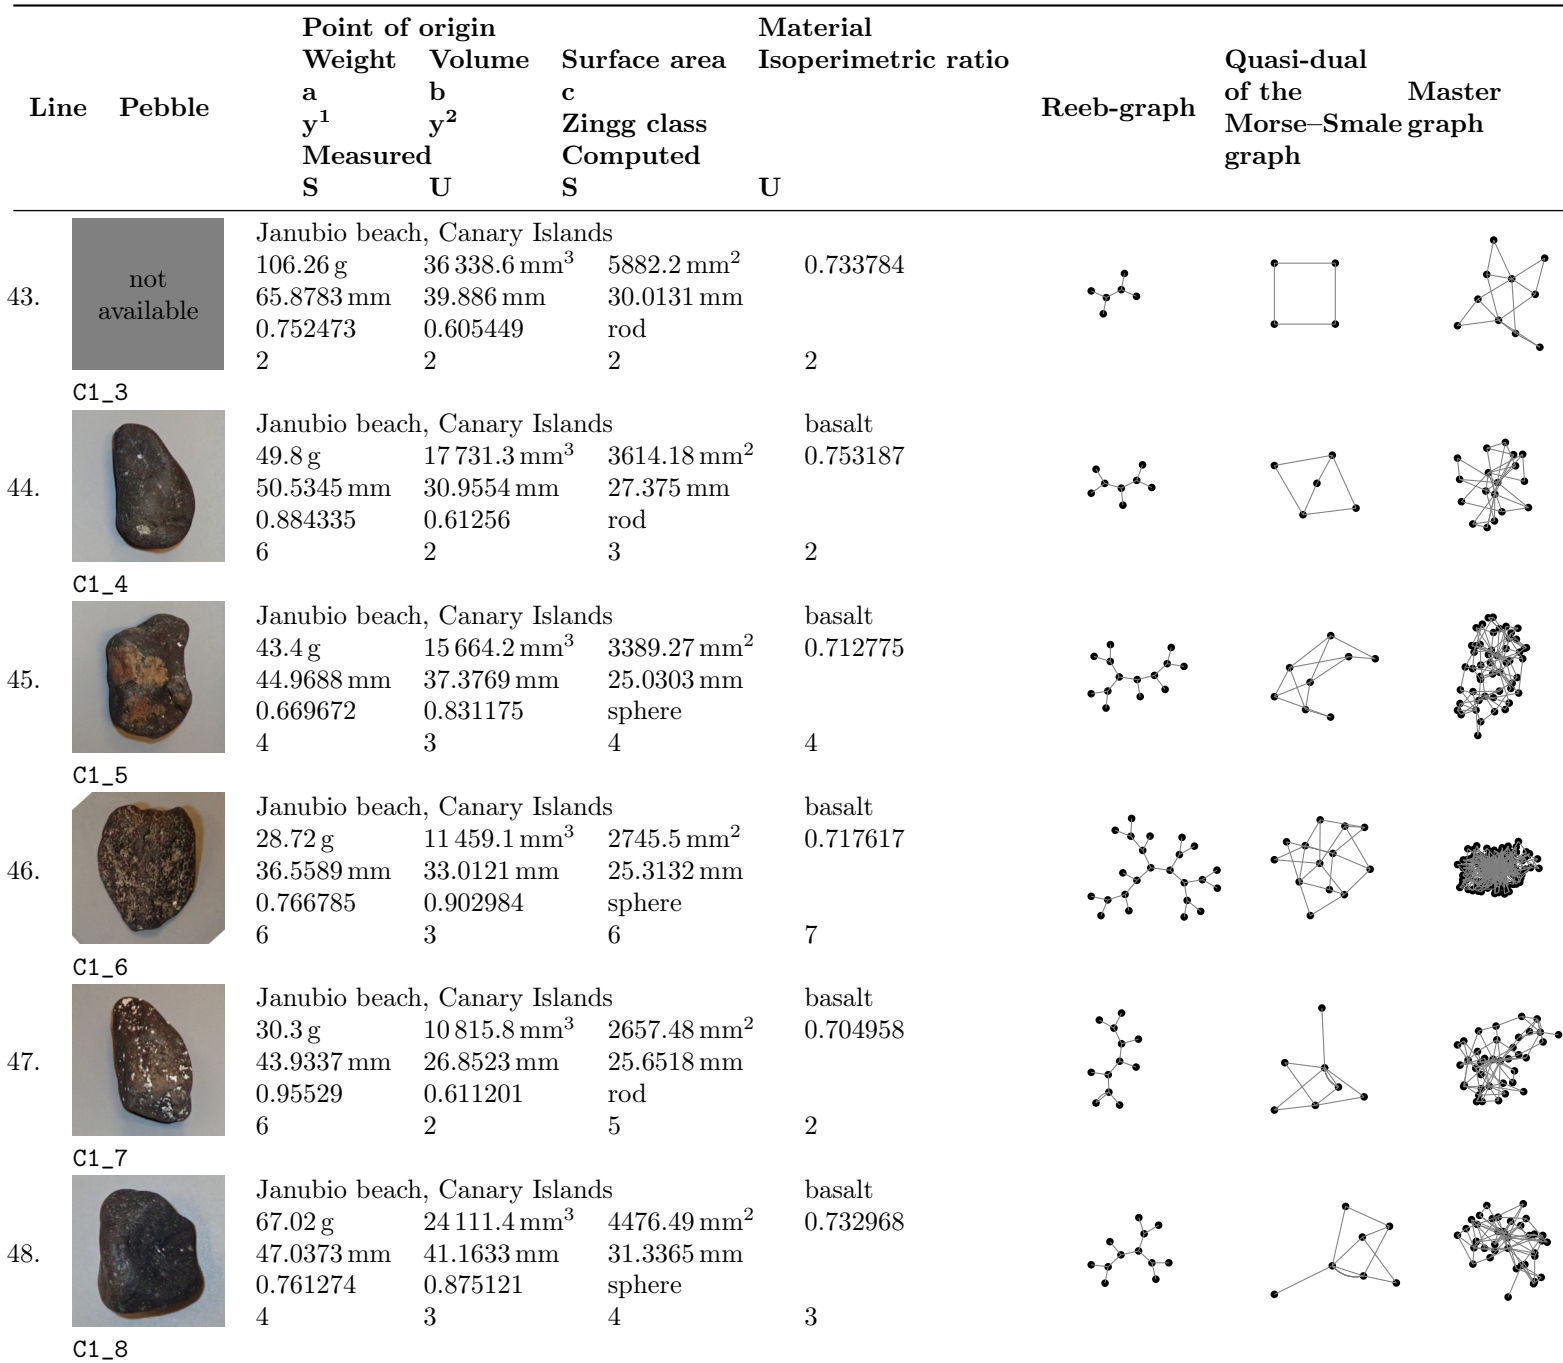   | 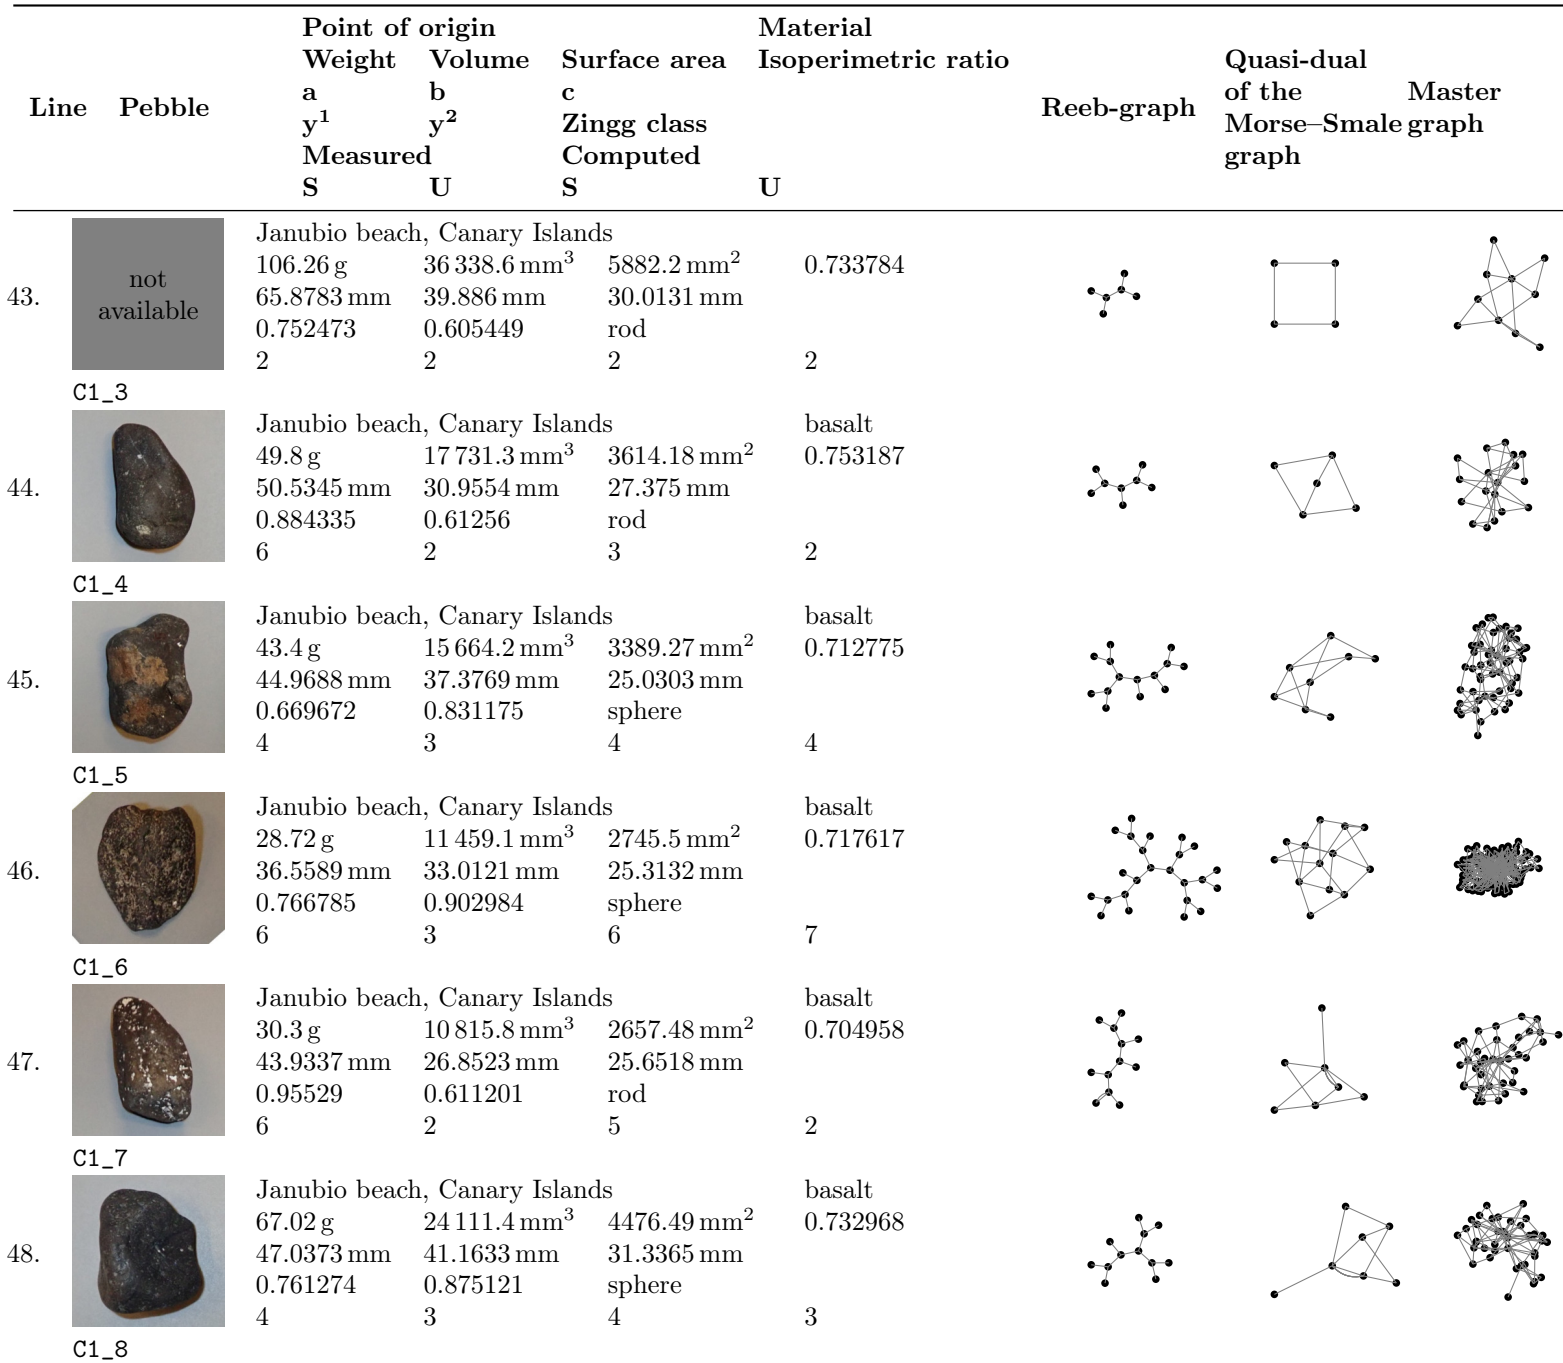   | 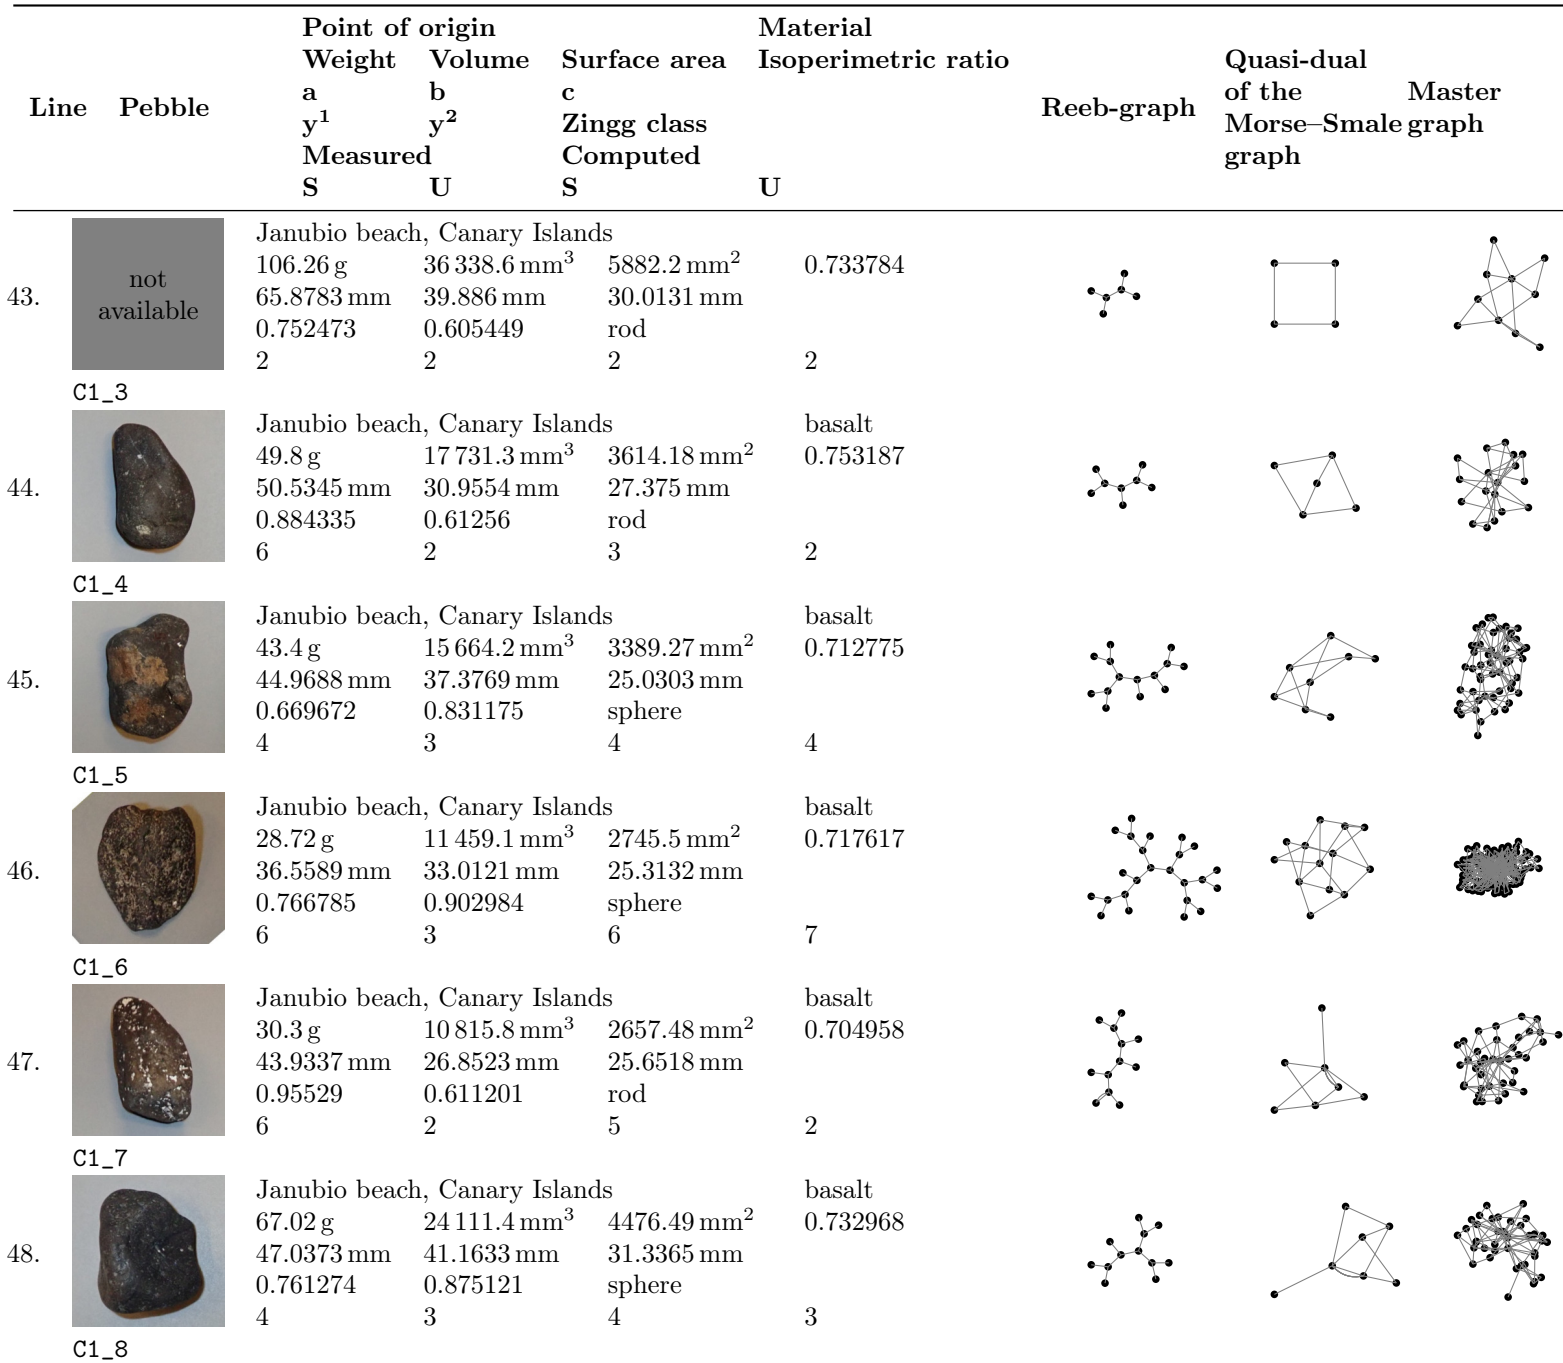   |
|      |                                                                                     | 43.4 g                        | 15 664.2 mm <sup>3</sup> | 3389.27 mm <sup>2</sup> | 0.712775 |                     |                                                                                       |                                                                                       |                                                                                       |
|      |                                                                                     | 44.9688 mm                    | 37.3769 mm               | 25.0303 mm              |          |                     |                                                                                       |                                                                                       |                                                                                       |
|      |                                                                                     | 0.669672                      | 0.831175                 | sphere                  |          |                     |                                                                                       |                                                                                       |                                                                                       |
|      |                                                                                     | 4                             | 3                        | 4                       | 4        |                     |                                                                                       |                                                                                       |                                                                                       |
| C1_5 |                                                                                     |                               |                          |                         |          |                     |                                                                                       |                                                                                       |                                                                                       |
| 46.  | 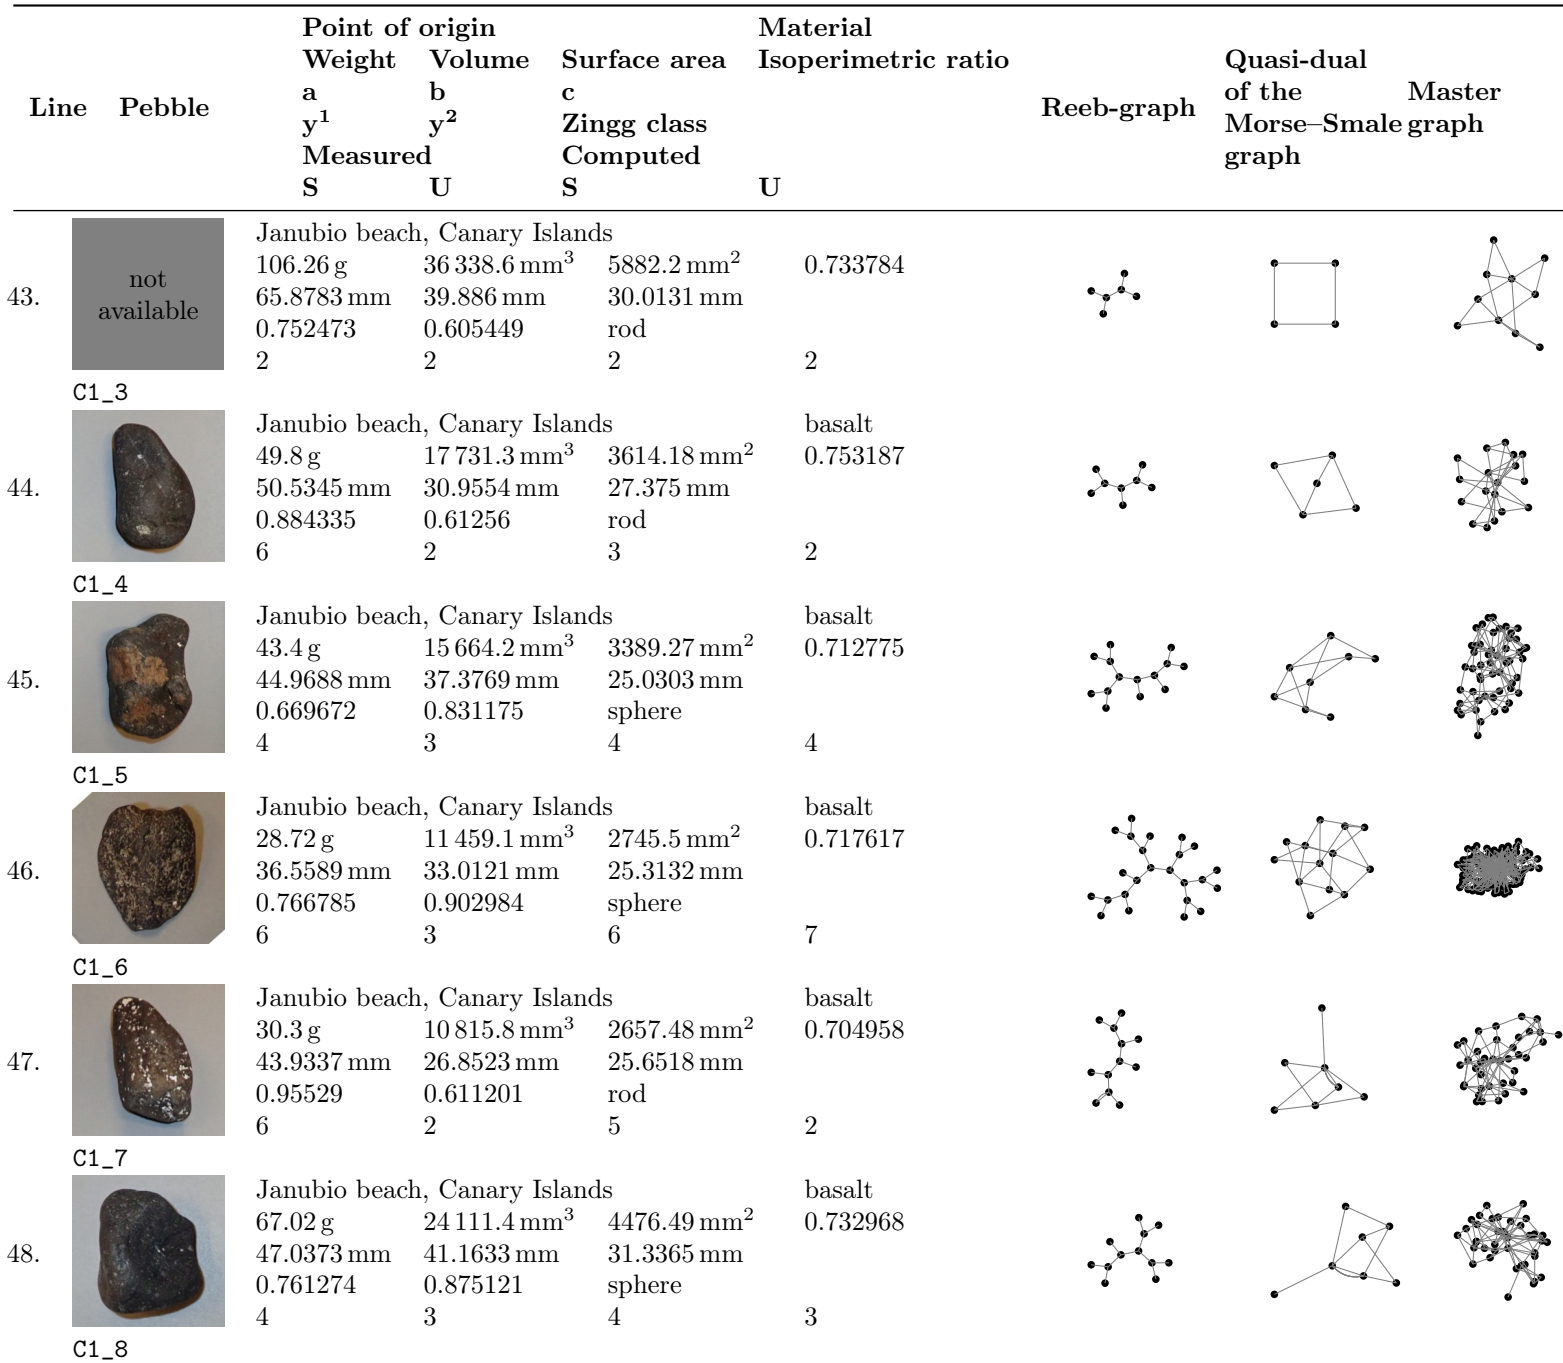  | Janubio beach, Canary Islands |                          |                         |          | basalt              | 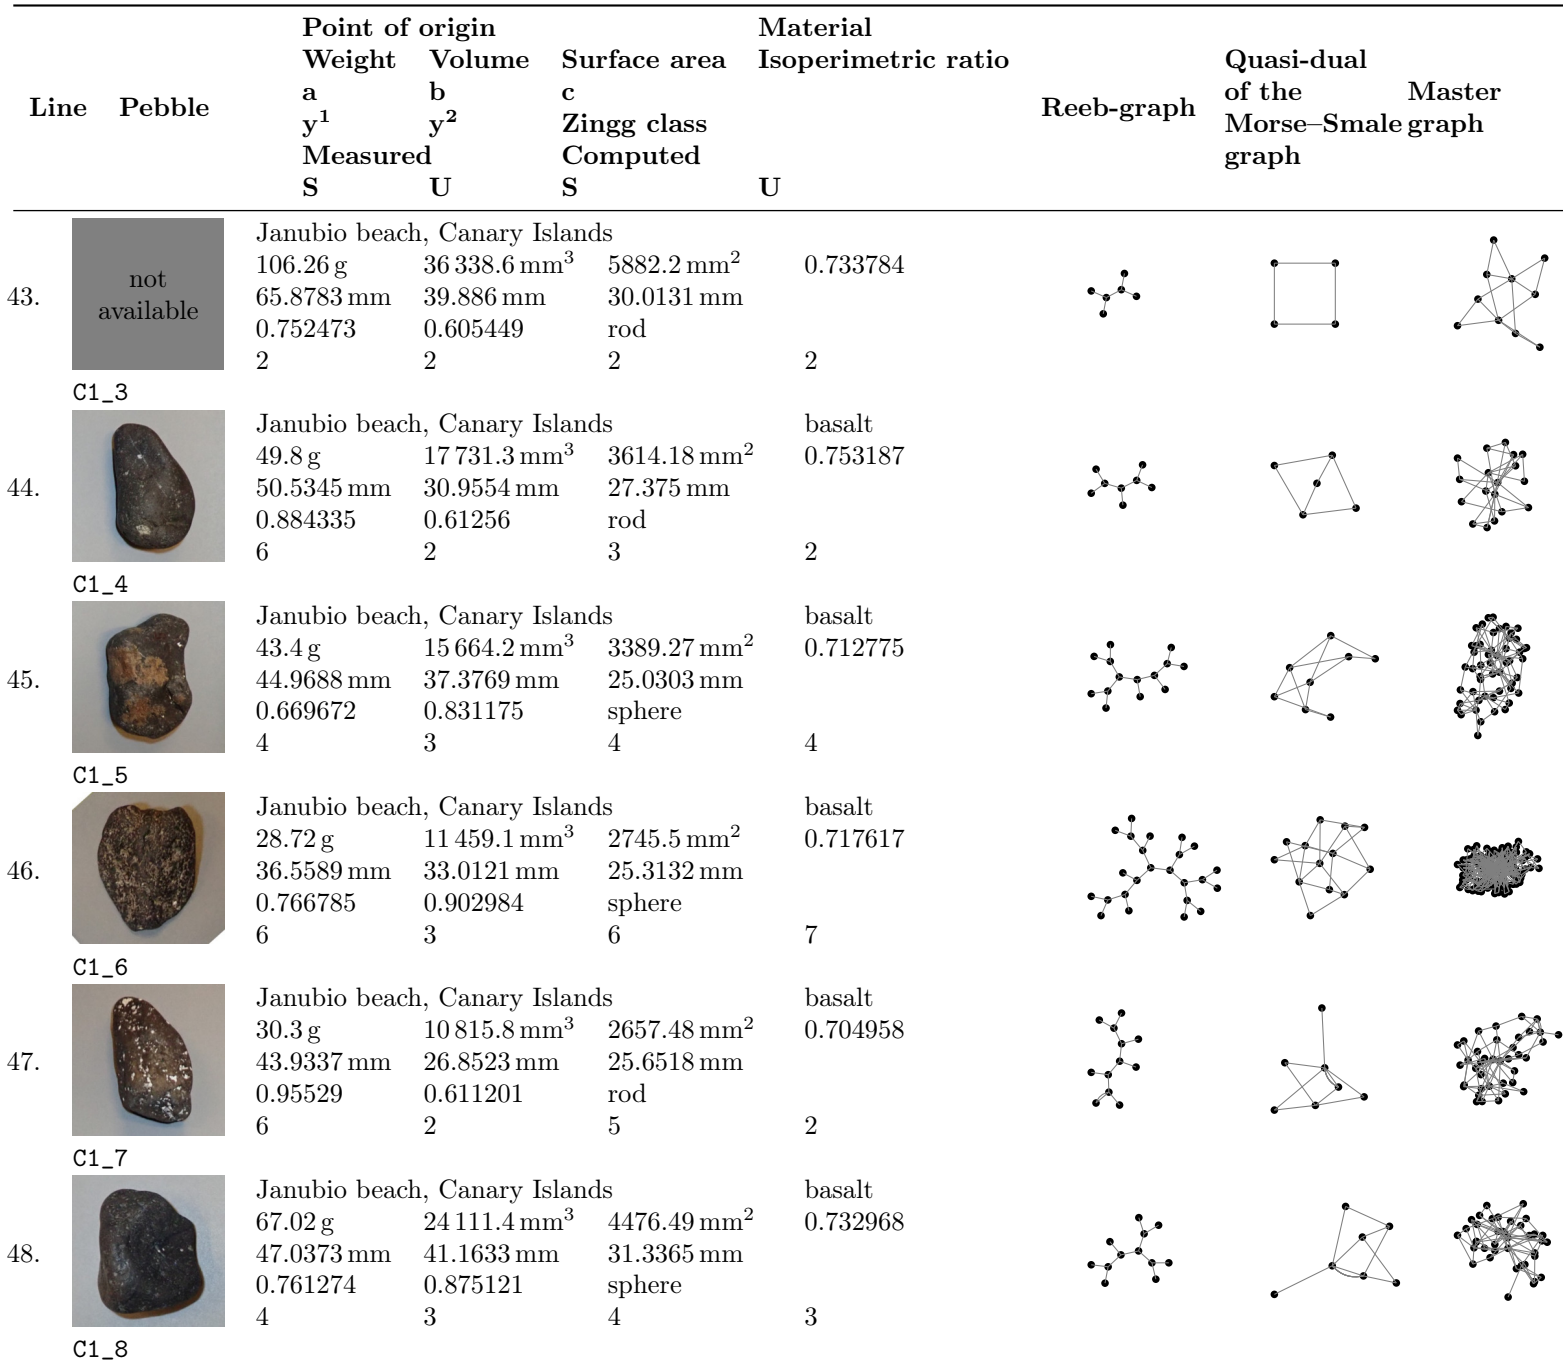  | 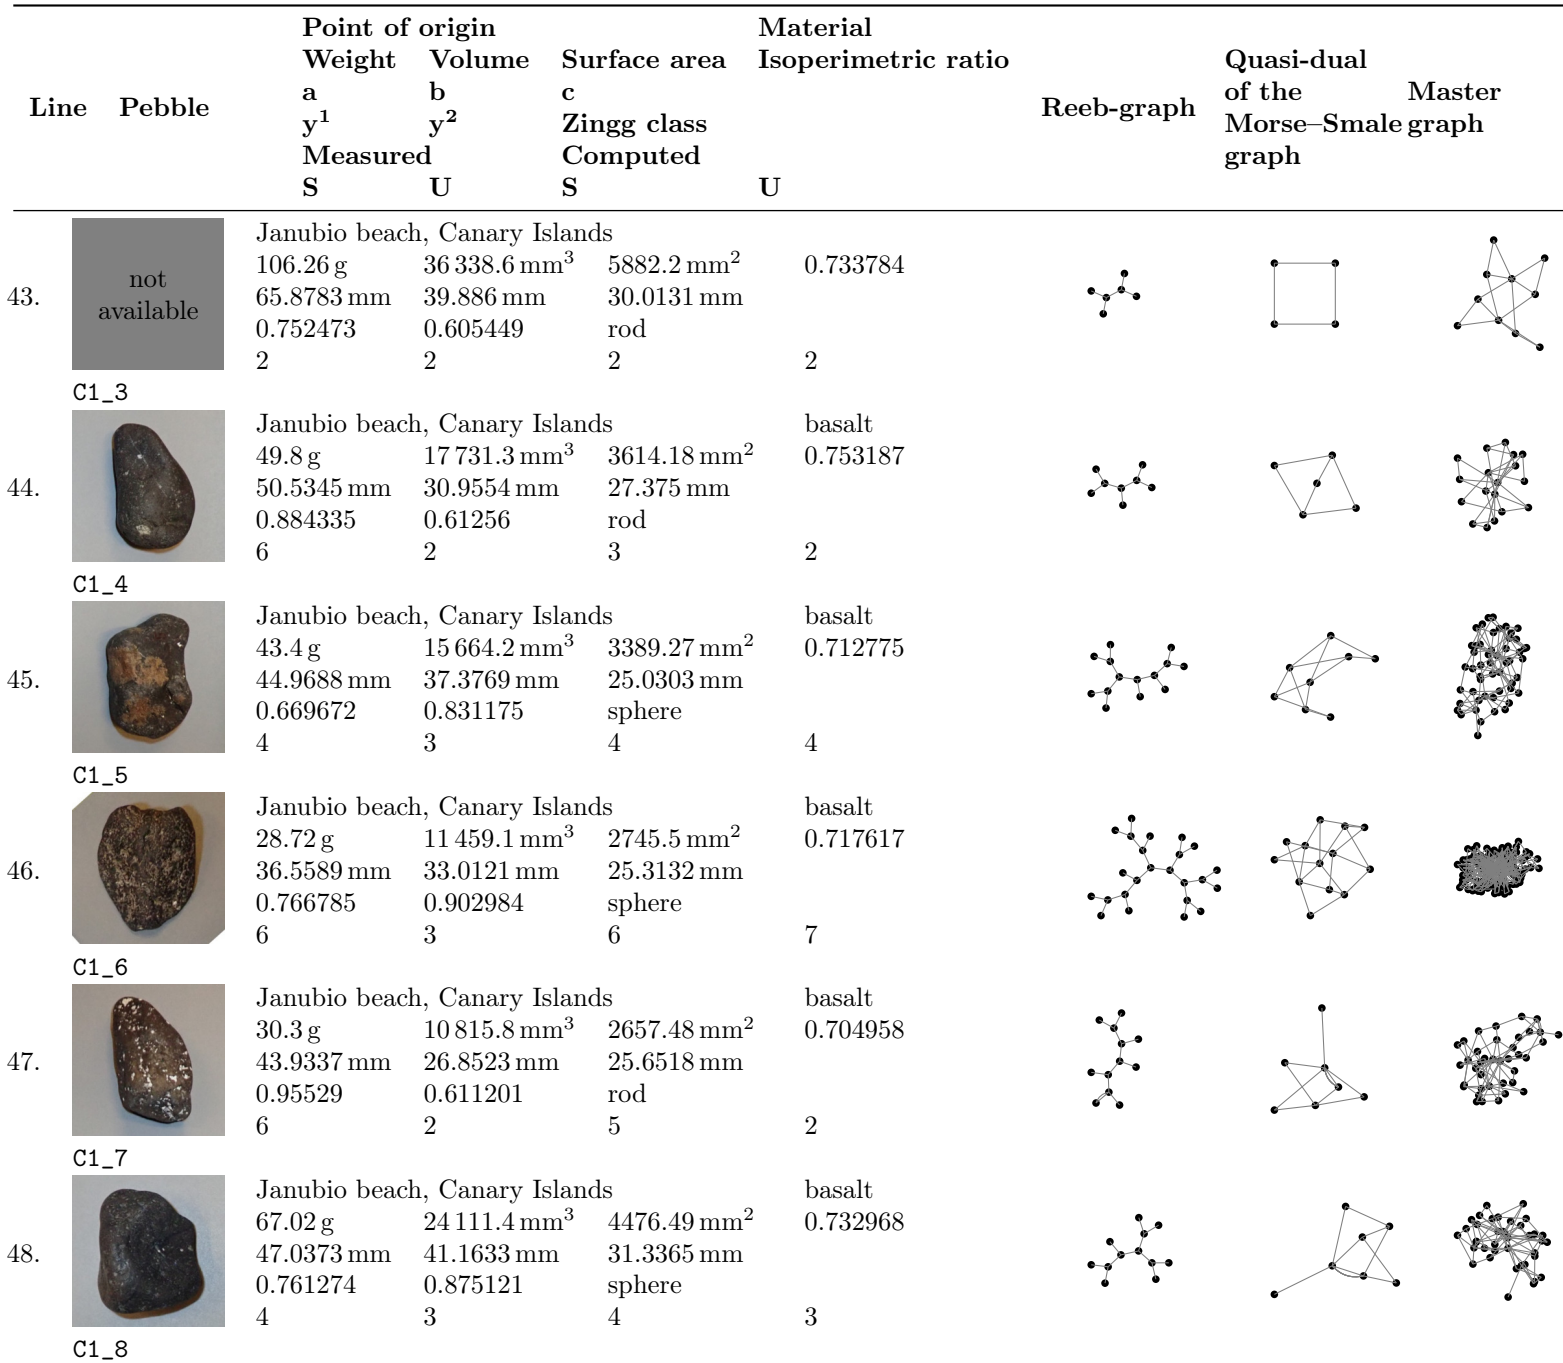  | 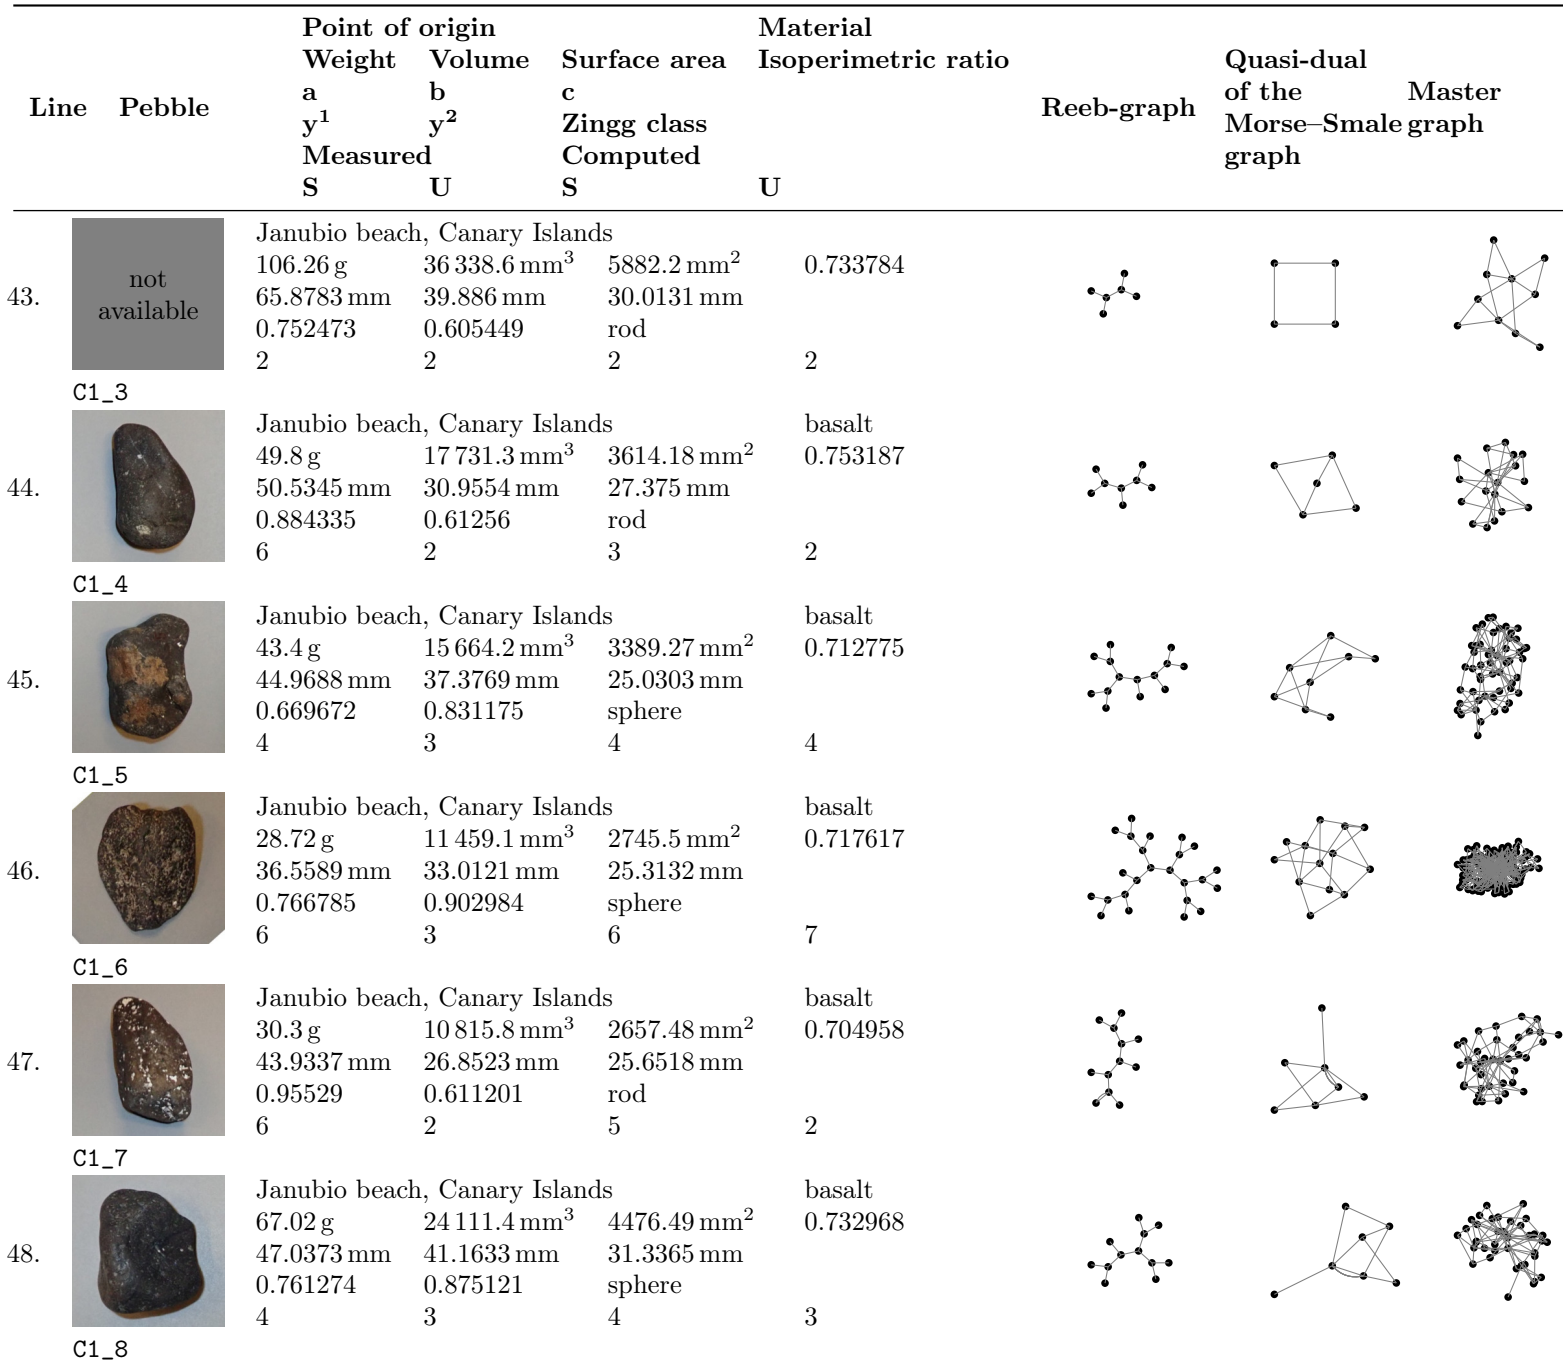  |
|      |                                                                                     | 28.72 g                       | 11 459.1 mm <sup>3</sup> | 2745.5 mm <sup>2</sup>  | 0.717617 |                     |                                                                                       |                                                                                       |                                                                                       |
|      |                                                                                     | 36.5589 mm                    | 33.0121 mm               | 25.3132 mm              |          |                     |                                                                                       |                                                                                       |                                                                                       |
|      |                                                                                     | 0.766785                      | 0.902984                 | sphere                  |          |                     |                                                                                       |                                                                                       |                                                                                       |
|      |                                                                                     | 6                             | 3                        | 6                       | 7        |                     |                                                                                       |                                                                                       |                                                                                       |
| C1_6 |                                                                                     |                               |                          |                         |          |                     |                                                                                       |                                                                                       |                                                                                       |
| 47.  | 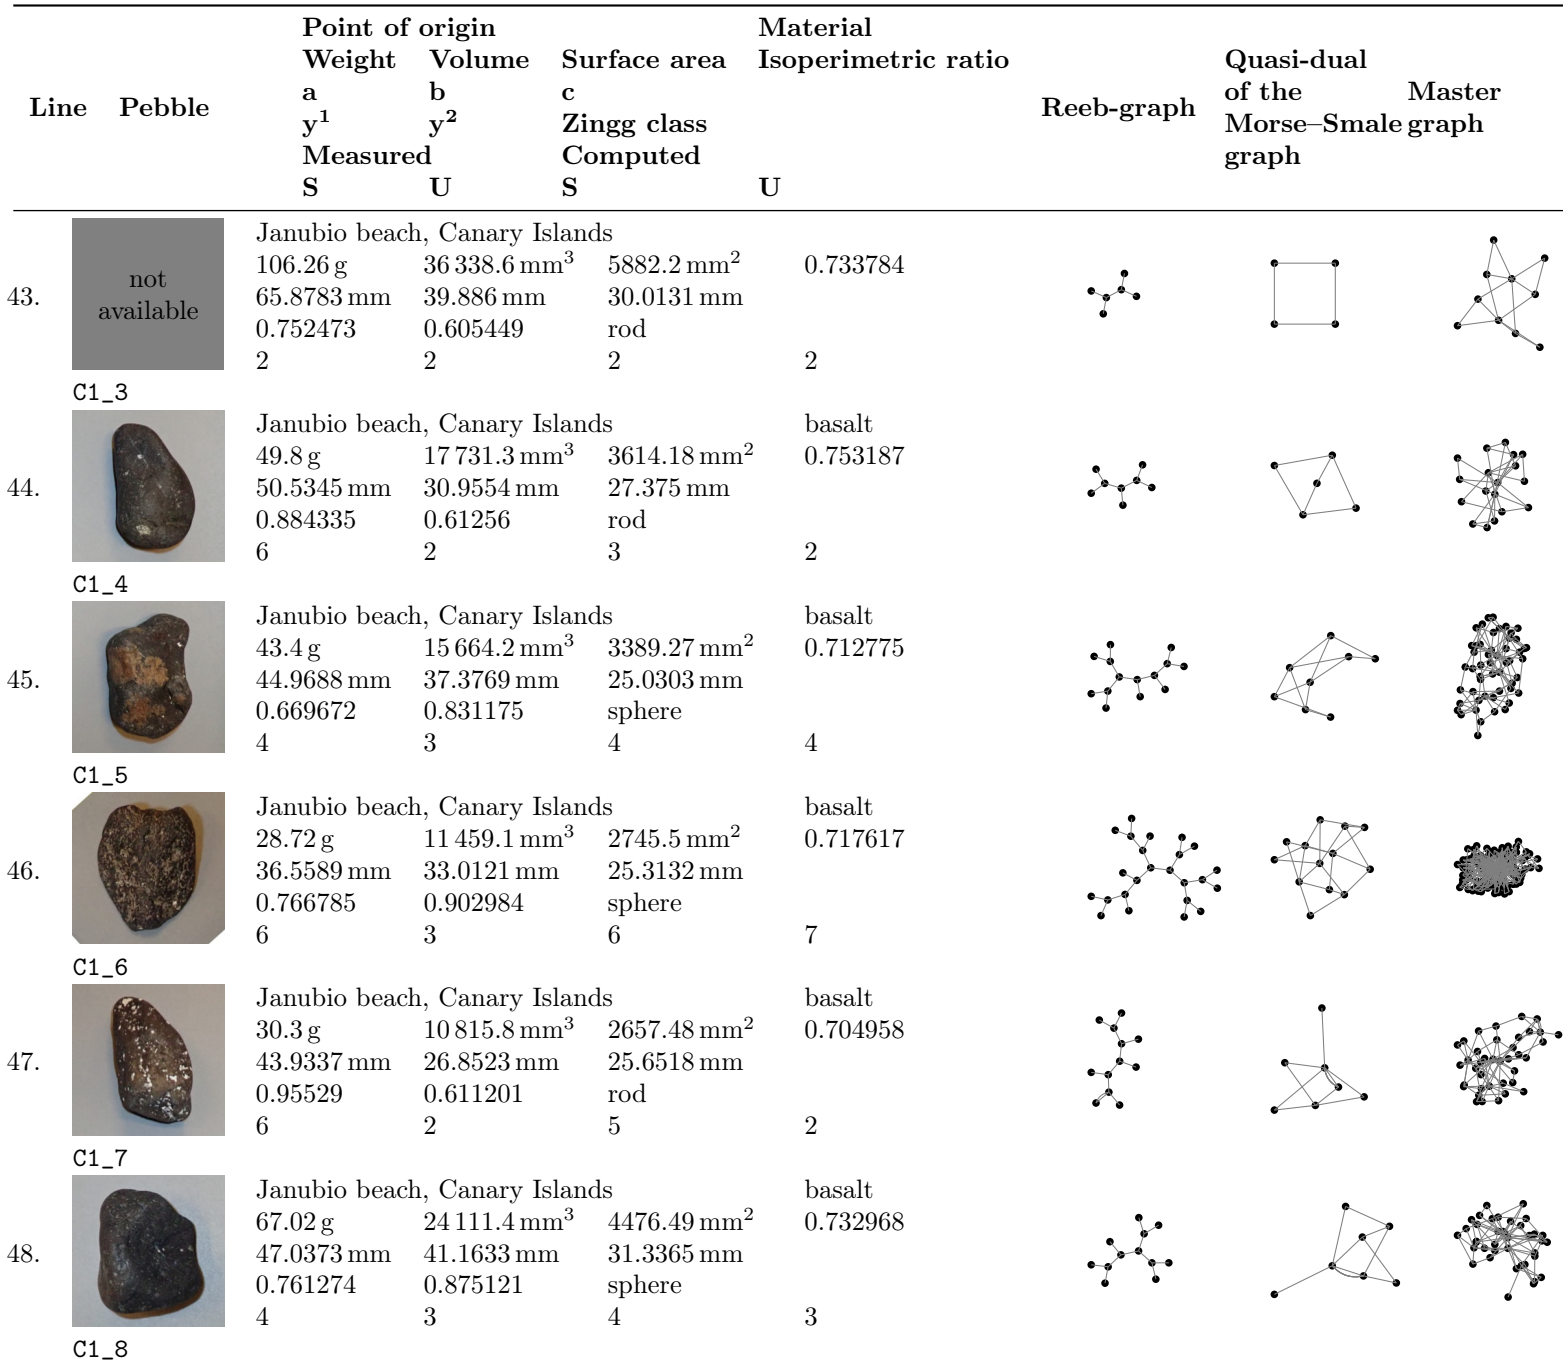 | Janubio beach, Canary Islands |                          |                         |          | basalt              | 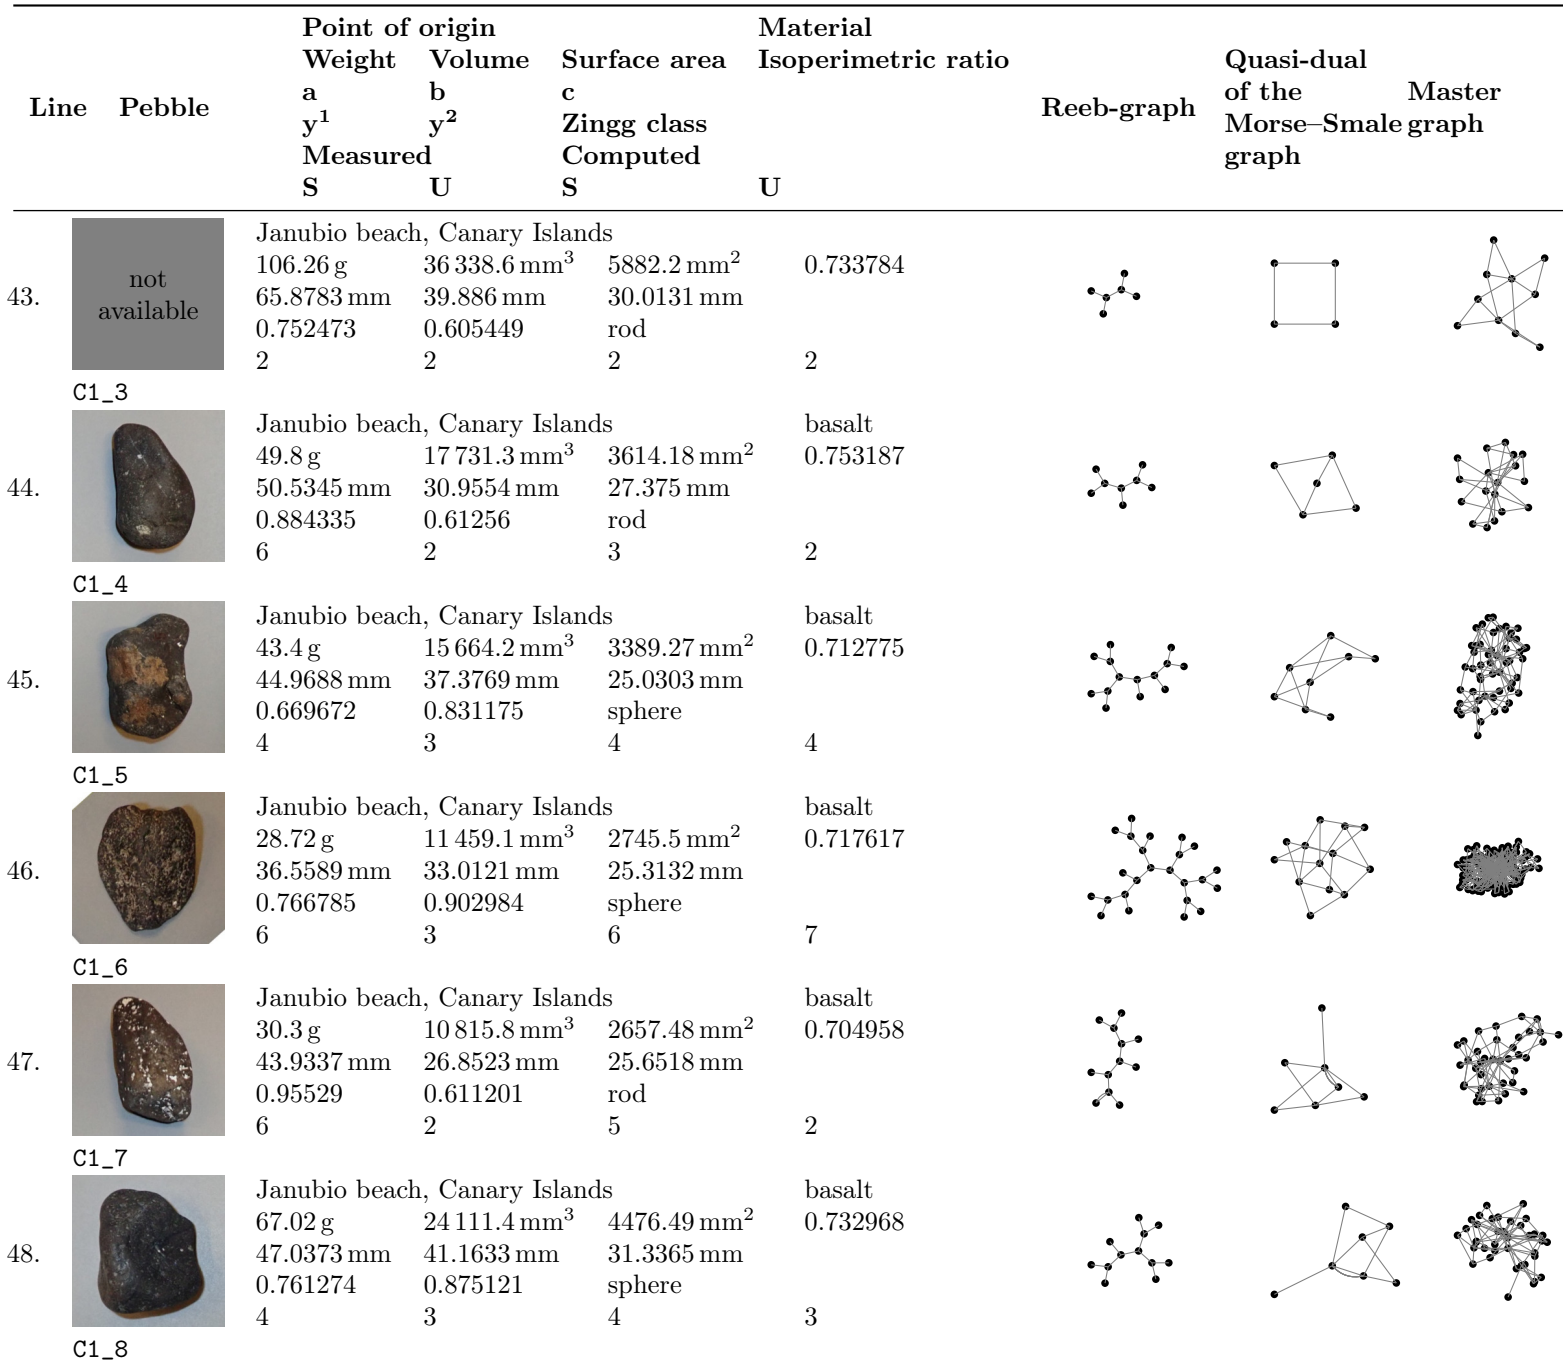 | 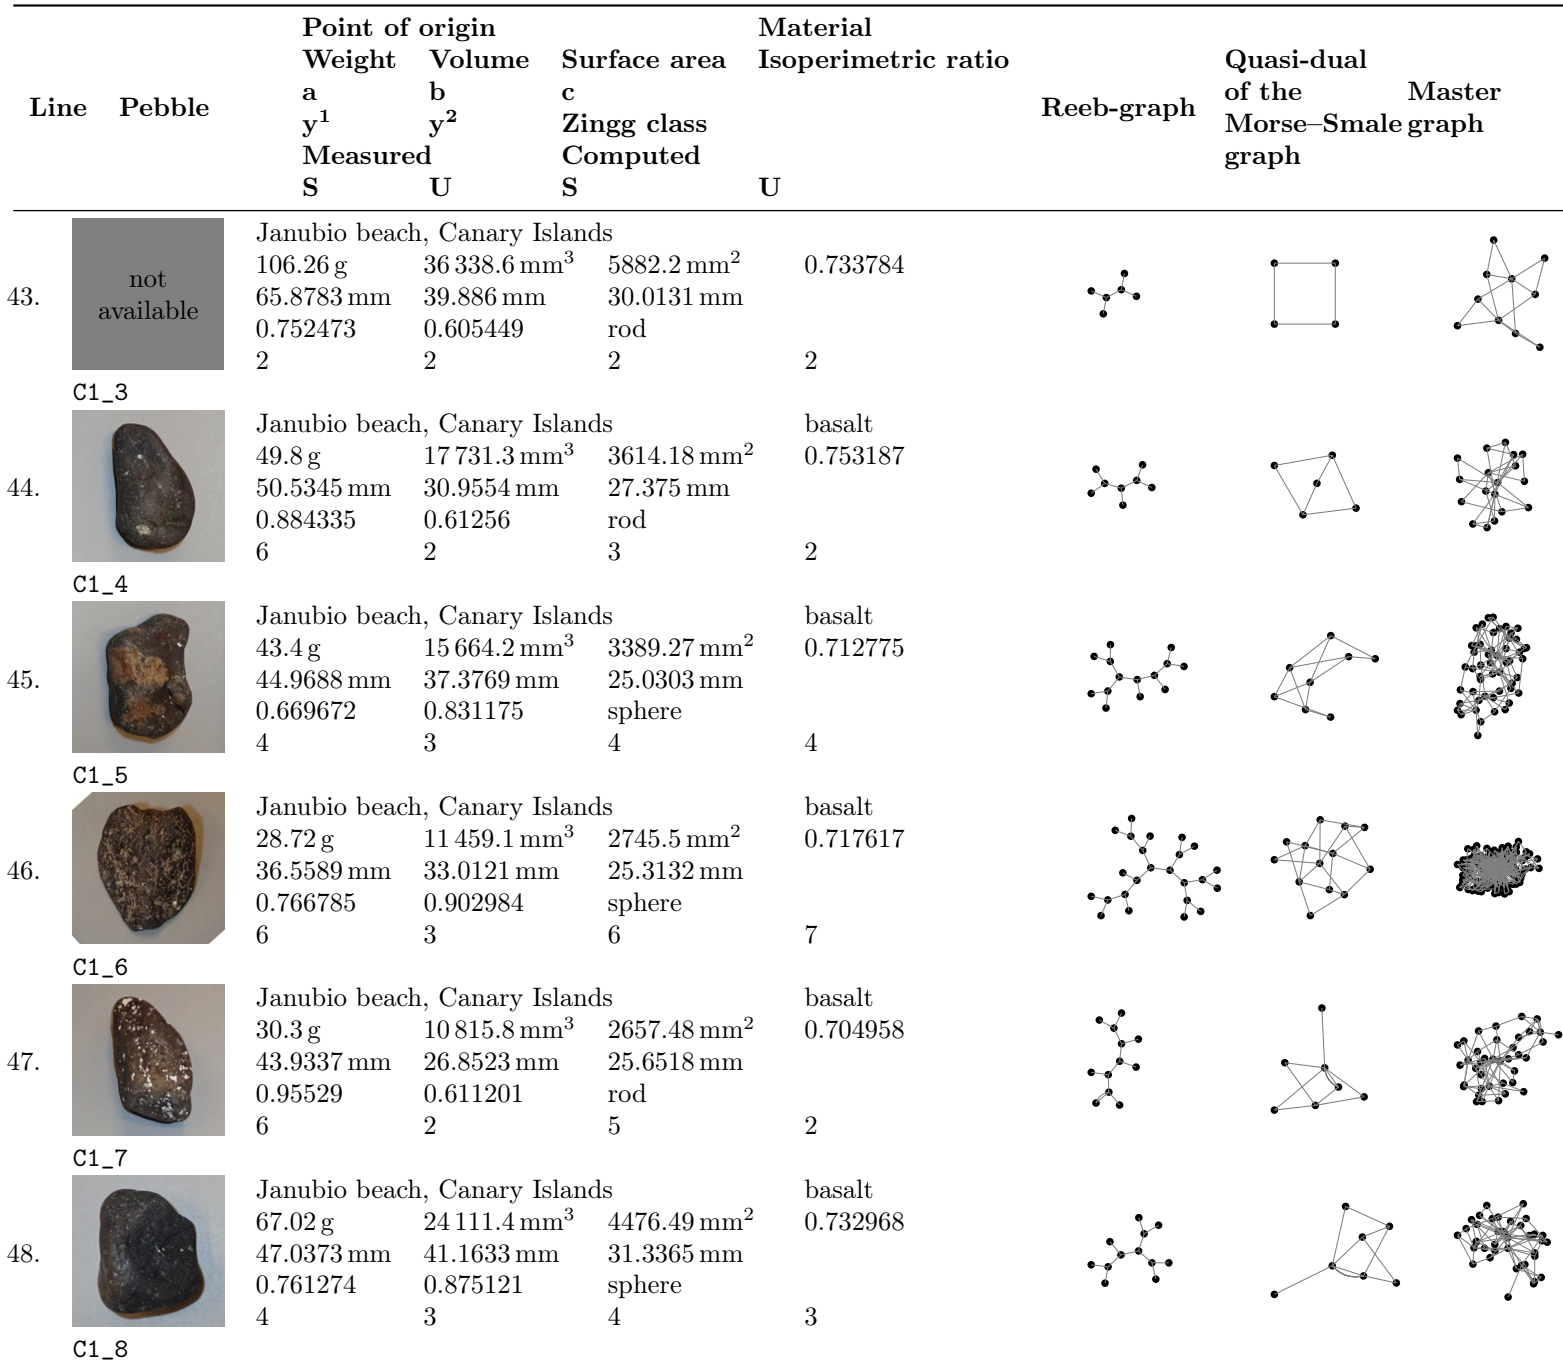 | 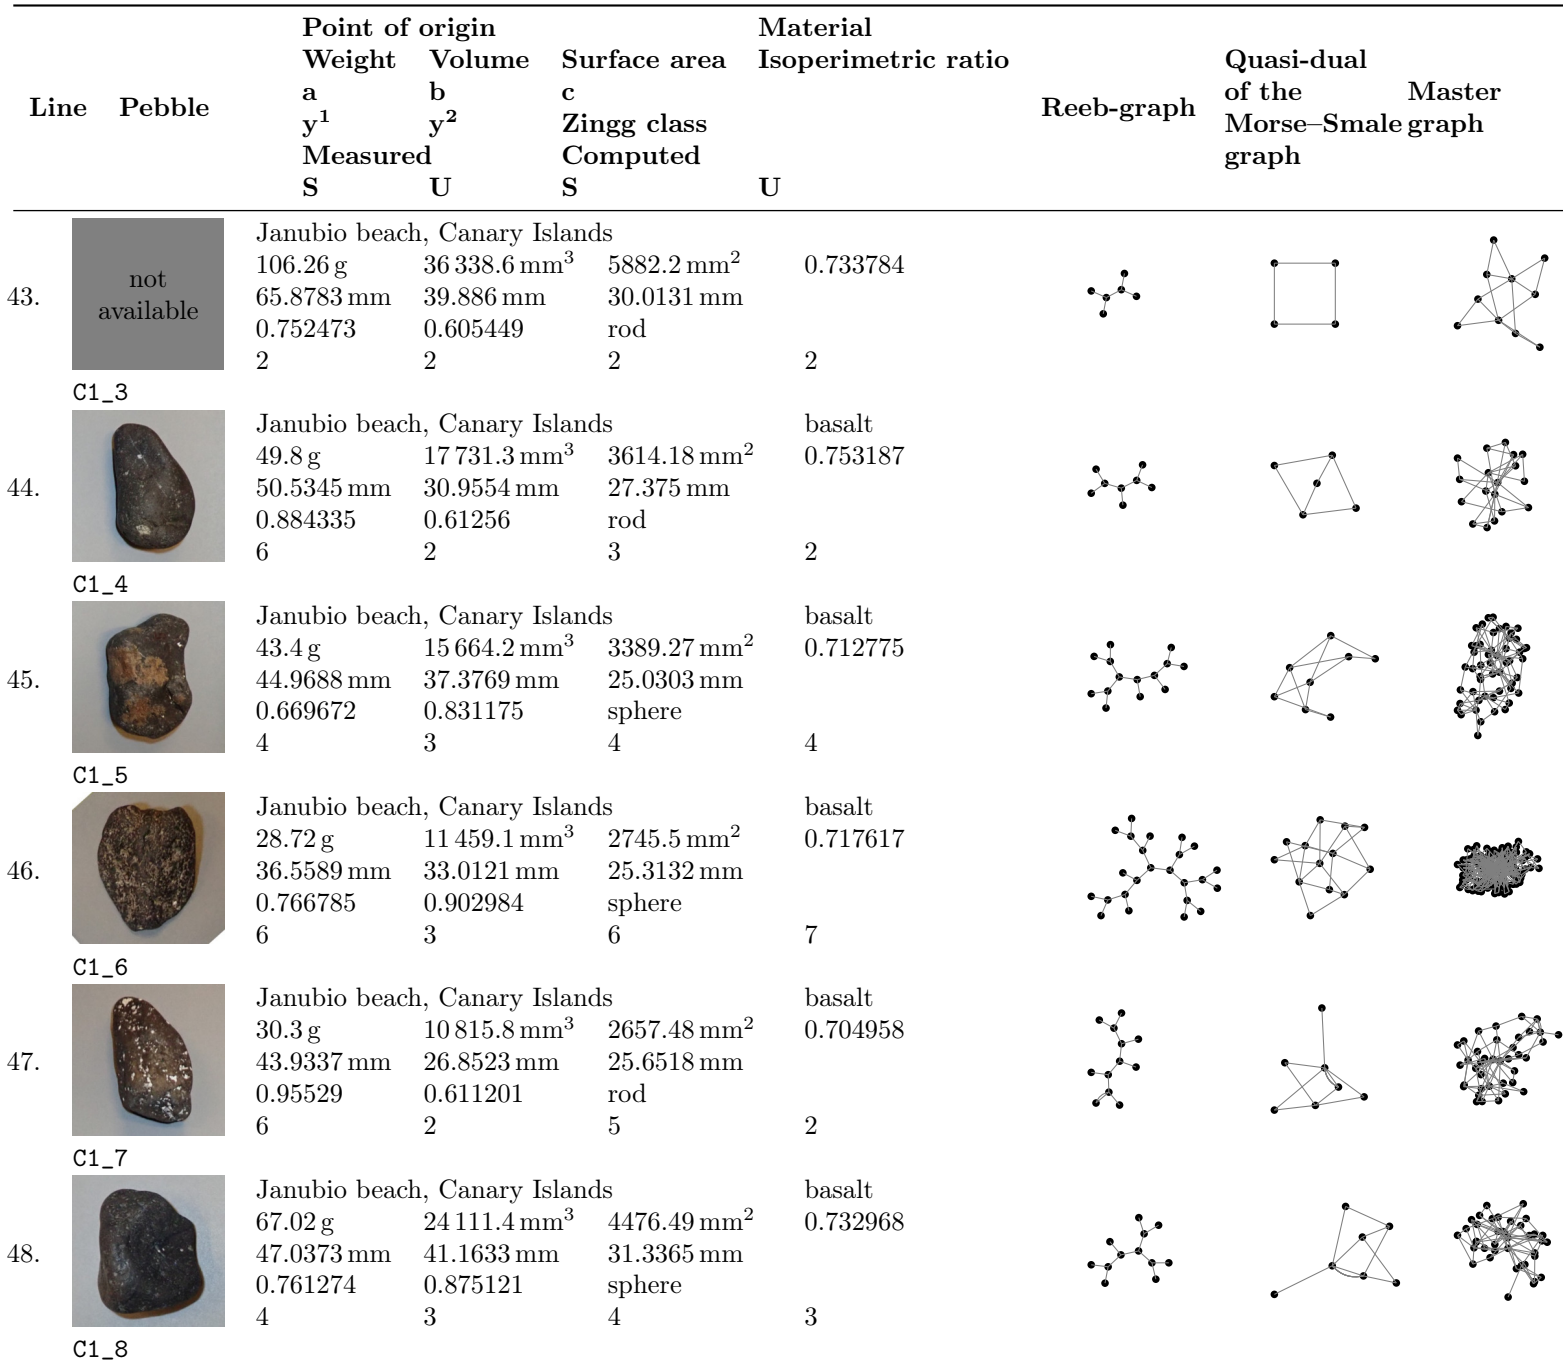 |
|      |                                                                                     | 30.3 g                        | 10 815.8 mm <sup>3</sup> | 2657.48 mm <sup>2</sup> | 0.704958 |                     |                                                                                       |                                                                                       |                                                                                       |
|      |                                                                                     | 43.9337 mm                    | 26.8523 mm               | 25.6518 mm              |          |                     |                                                                                       |                                                                                       |                                                                                       |
|      |                                                                                     | 0.95529                       | 0.611201                 | rod                     |          |                     |                                                                                       |                                                                                       |                                                                                       |
|      |                                                                                     | 6                             | 2                        | 5                       | 2        |                     |                                                                                       |                                                                                       |                                                                                       |
| C1_7 |                                                                                     |                               |                          |                         |          |                     |                                                                                       |                                                                                       |                                                                                       |
| 48.  | 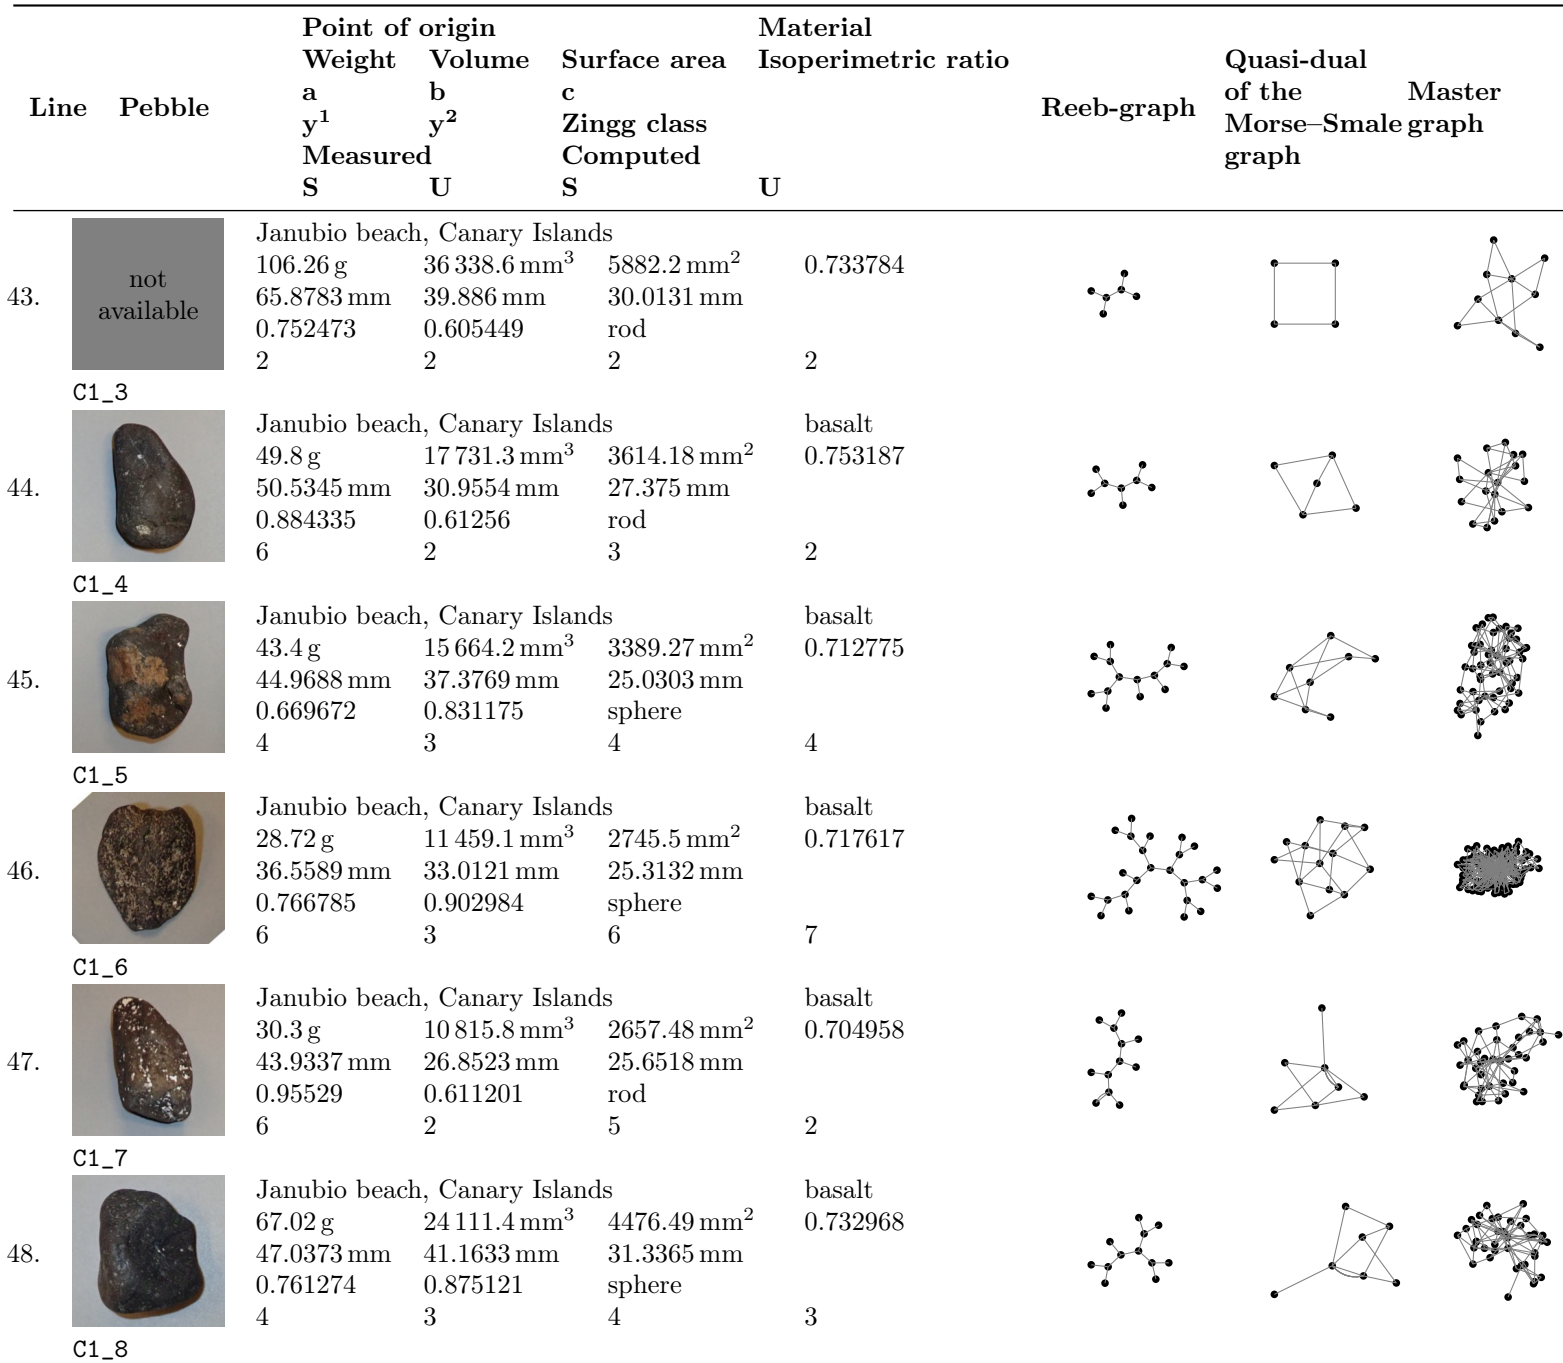 | Janubio beach, Canary Islands |                          |                         |          | basalt              | 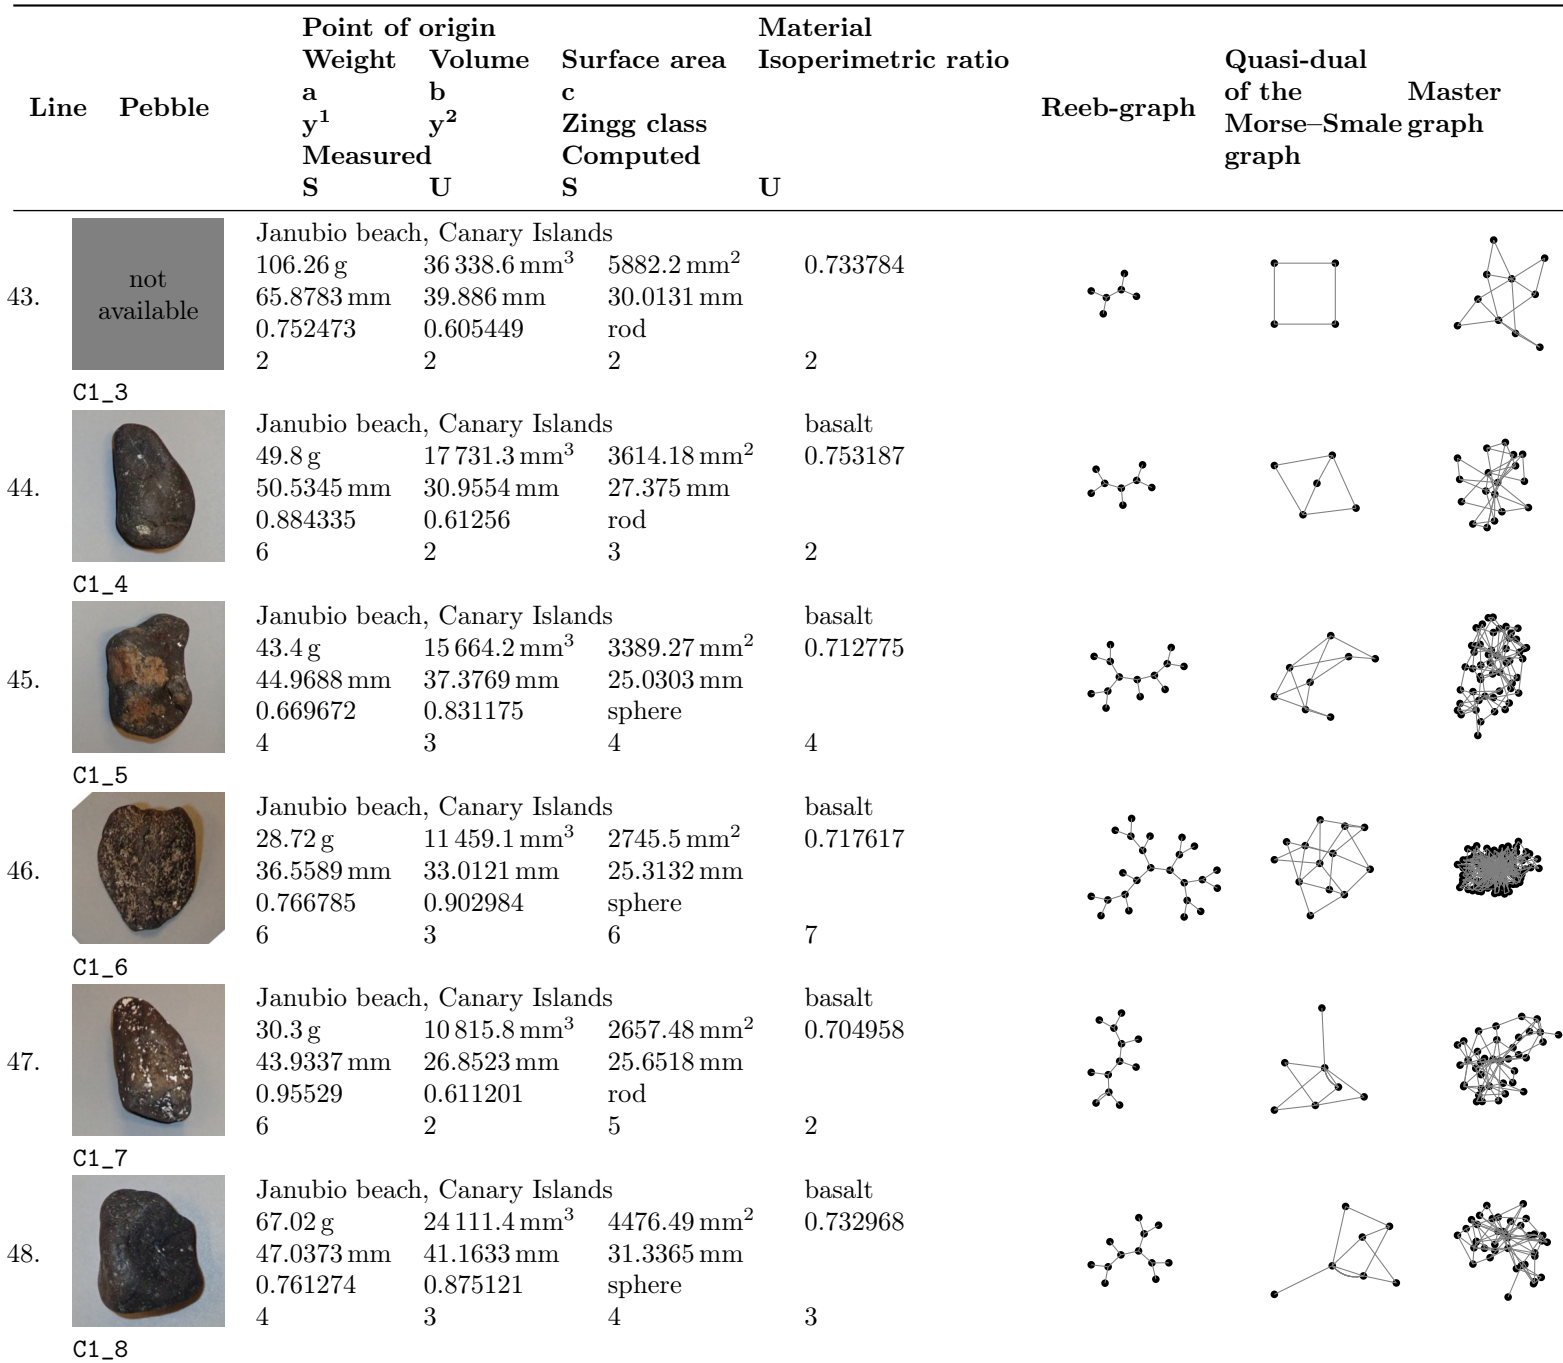 | 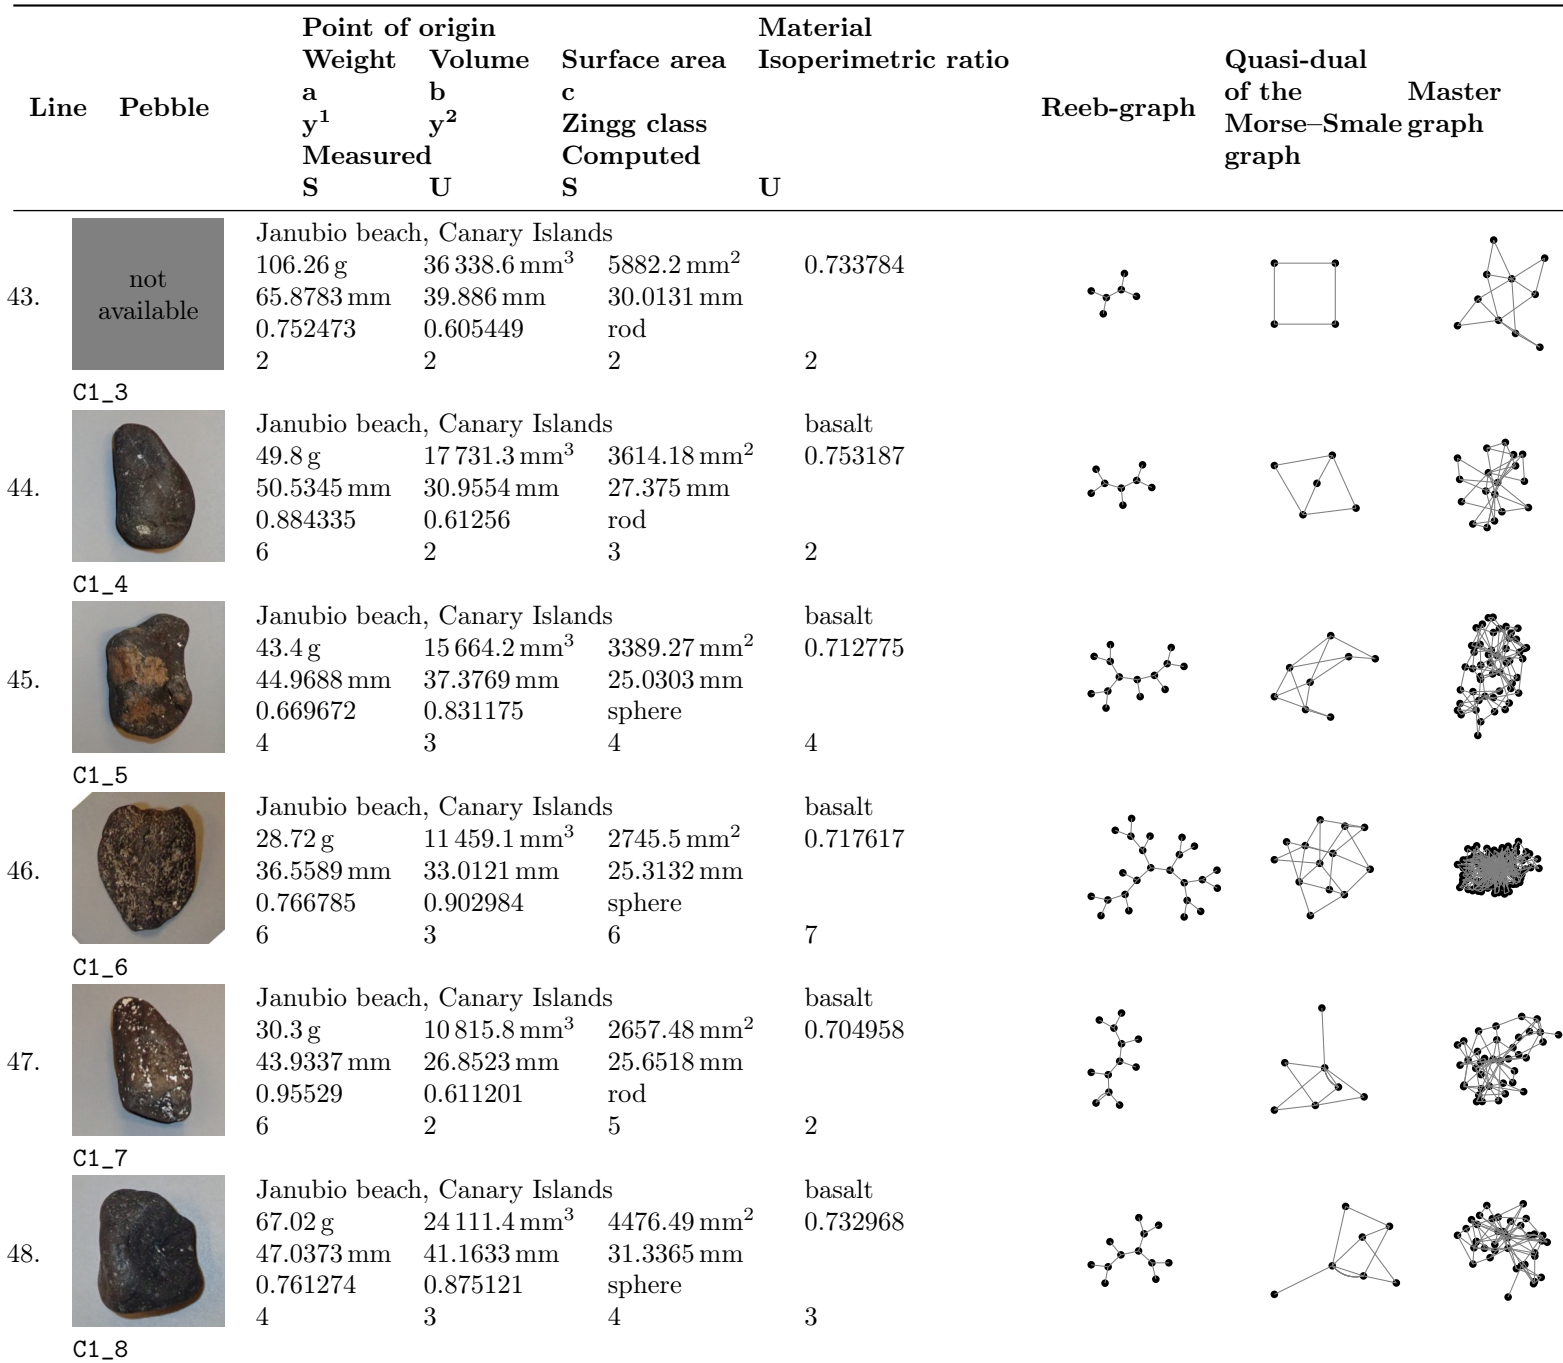 | 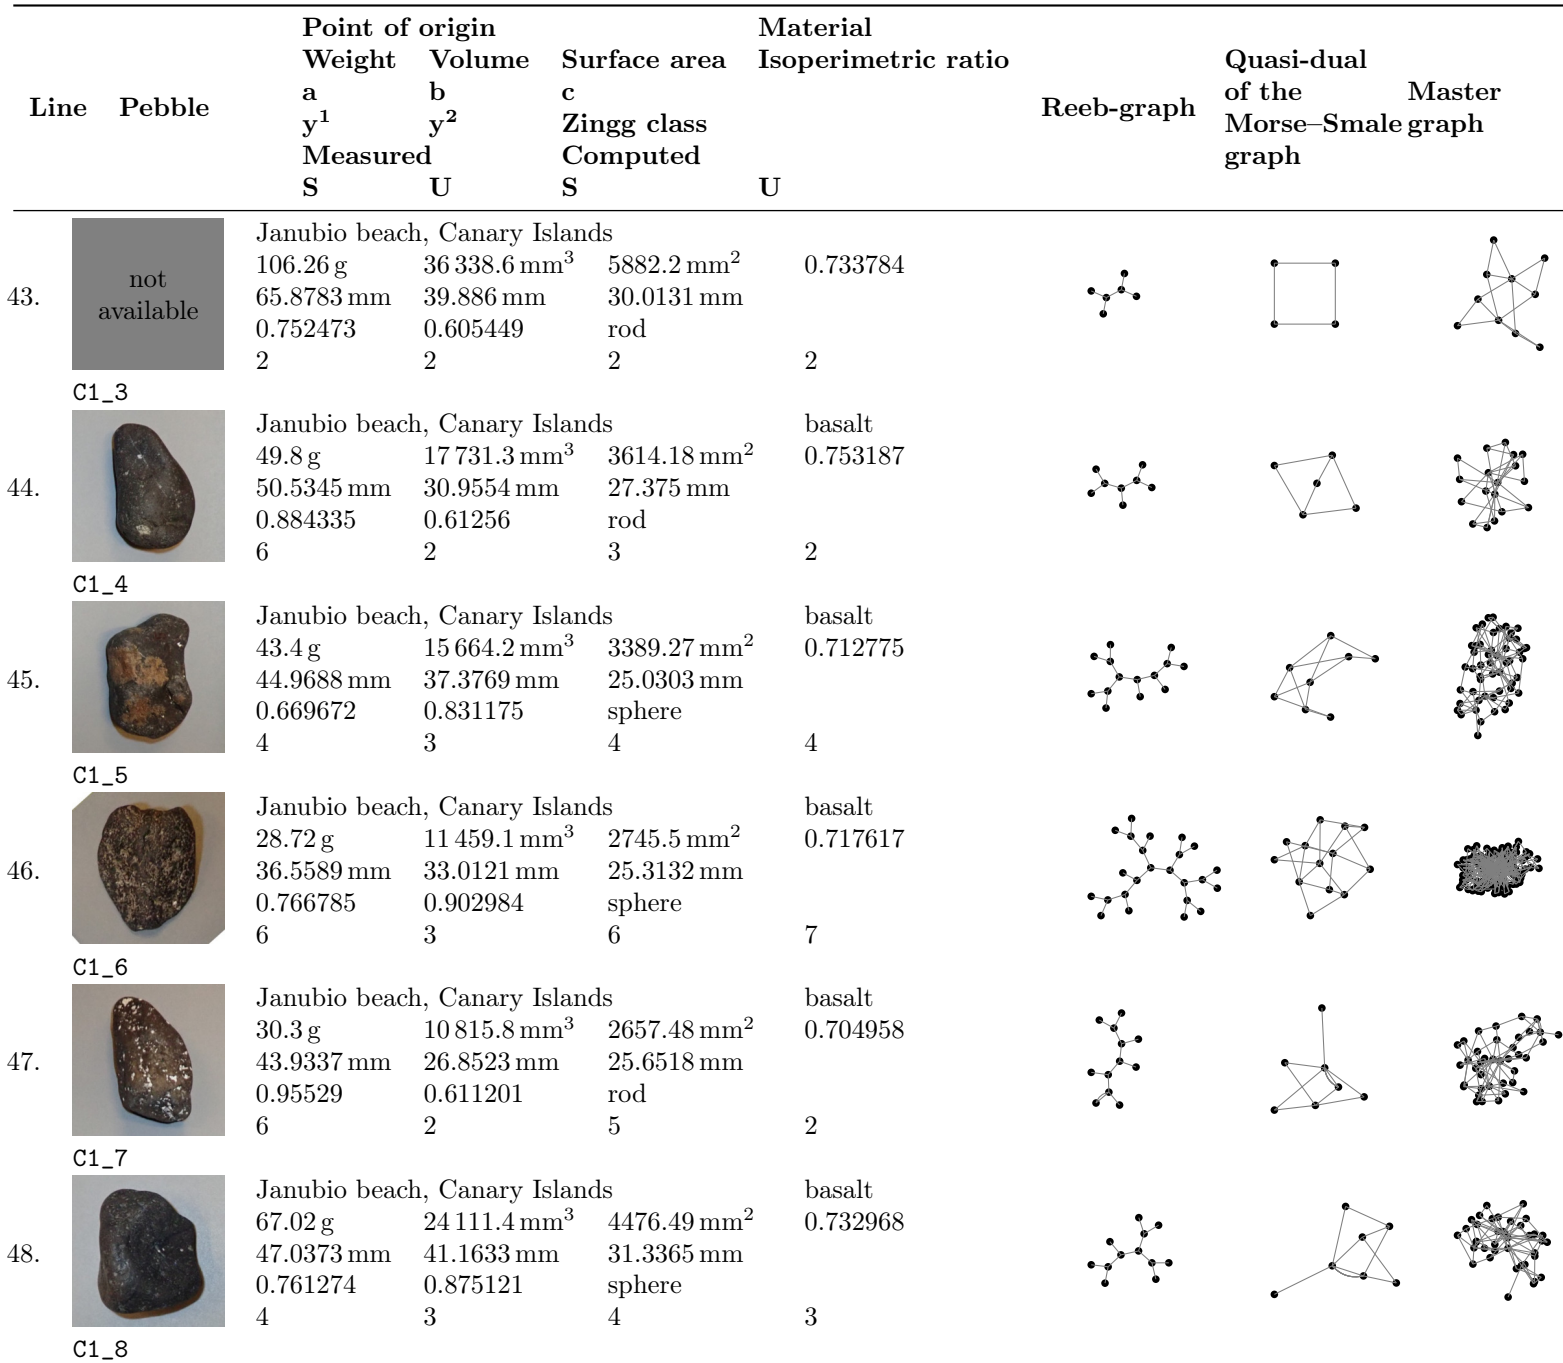 |
|      |                                                                                     | 67.02 g                       | 24 111.4 mm <sup>3</sup> | 4476.49 mm <sup>2</sup> | 0.732968 |                     |                                                                                       |                                                                                       |                                                                                       |
|      |                                                                                     | 47.0373 mm                    | 41.1633 mm               | 31.3365 mm              |          |                     |                                                                                       |                                                                                       |                                                                                       |
|      |                                                                                     | 0.761274                      | 0.875121                 | sphere                  |          |                     |                                                                                       |                                                                                       |                                                                                       |
|      |                                                                                     | 4                             | 3                        | 4                       | 3        |                     |                                                                                       |                                                                                       |                                                                                       |
| C1_8 |                                                                                     |                               |                          |                         |          |                     |                                                                                       |                                                                                       |                                                                                       |

| Line | Pebble                                                                              | Point of origin                      |                          | Surface area<br>c<br>Zingg class<br>Computed<br>S    | Material<br>Isoperimetric ratio<br>U | Reeb-graph                                                                            | Quasi-dual<br>of the<br>Morse–Smale<br>graph                                          | Master<br>graph                                                                       |
|------|-------------------------------------------------------------------------------------|--------------------------------------|--------------------------|------------------------------------------------------|--------------------------------------|---------------------------------------------------------------------------------------|---------------------------------------------------------------------------------------|---------------------------------------------------------------------------------------|
|      |                                                                                     | Weight                               | Volume                   |                                                      |                                      |                                                                                       |                                                                                       |                                                                                       |
|      |                                                                                     | a<br>y <sup>1</sup><br>Measured<br>S | b<br>y <sup>2</sup><br>U |                                                      |                                      |                                                                                       |                                                                                       |                                                                                       |
|      |                                                                                     |                                      |                          |                                                      |                                      |                                                                                       |                                                                                       |                                                                                       |
| 49.  | 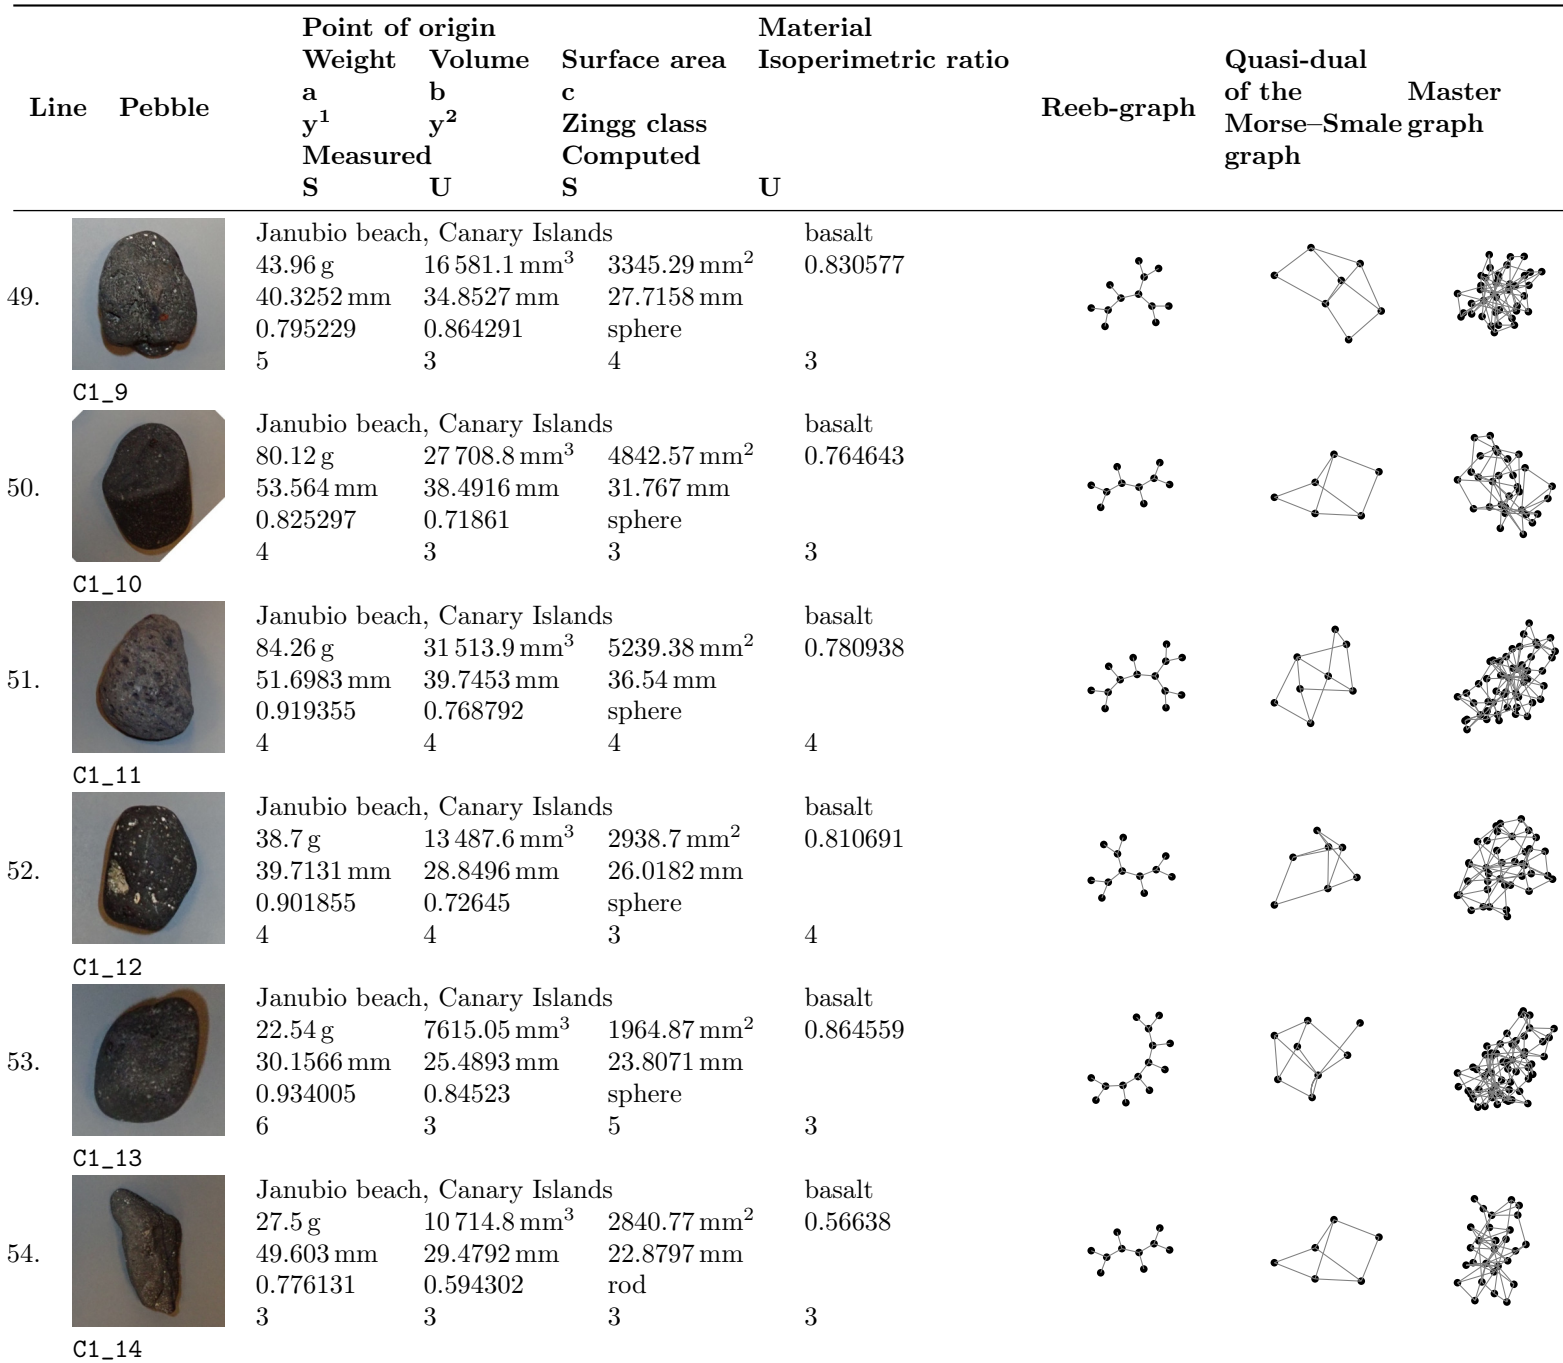   | Janubio beach, Canary Islands        |                          | 3345.29 mm <sup>2</sup><br>27.7158 mm<br>sphere<br>4 | basalt<br>0.830577<br><br>3          | 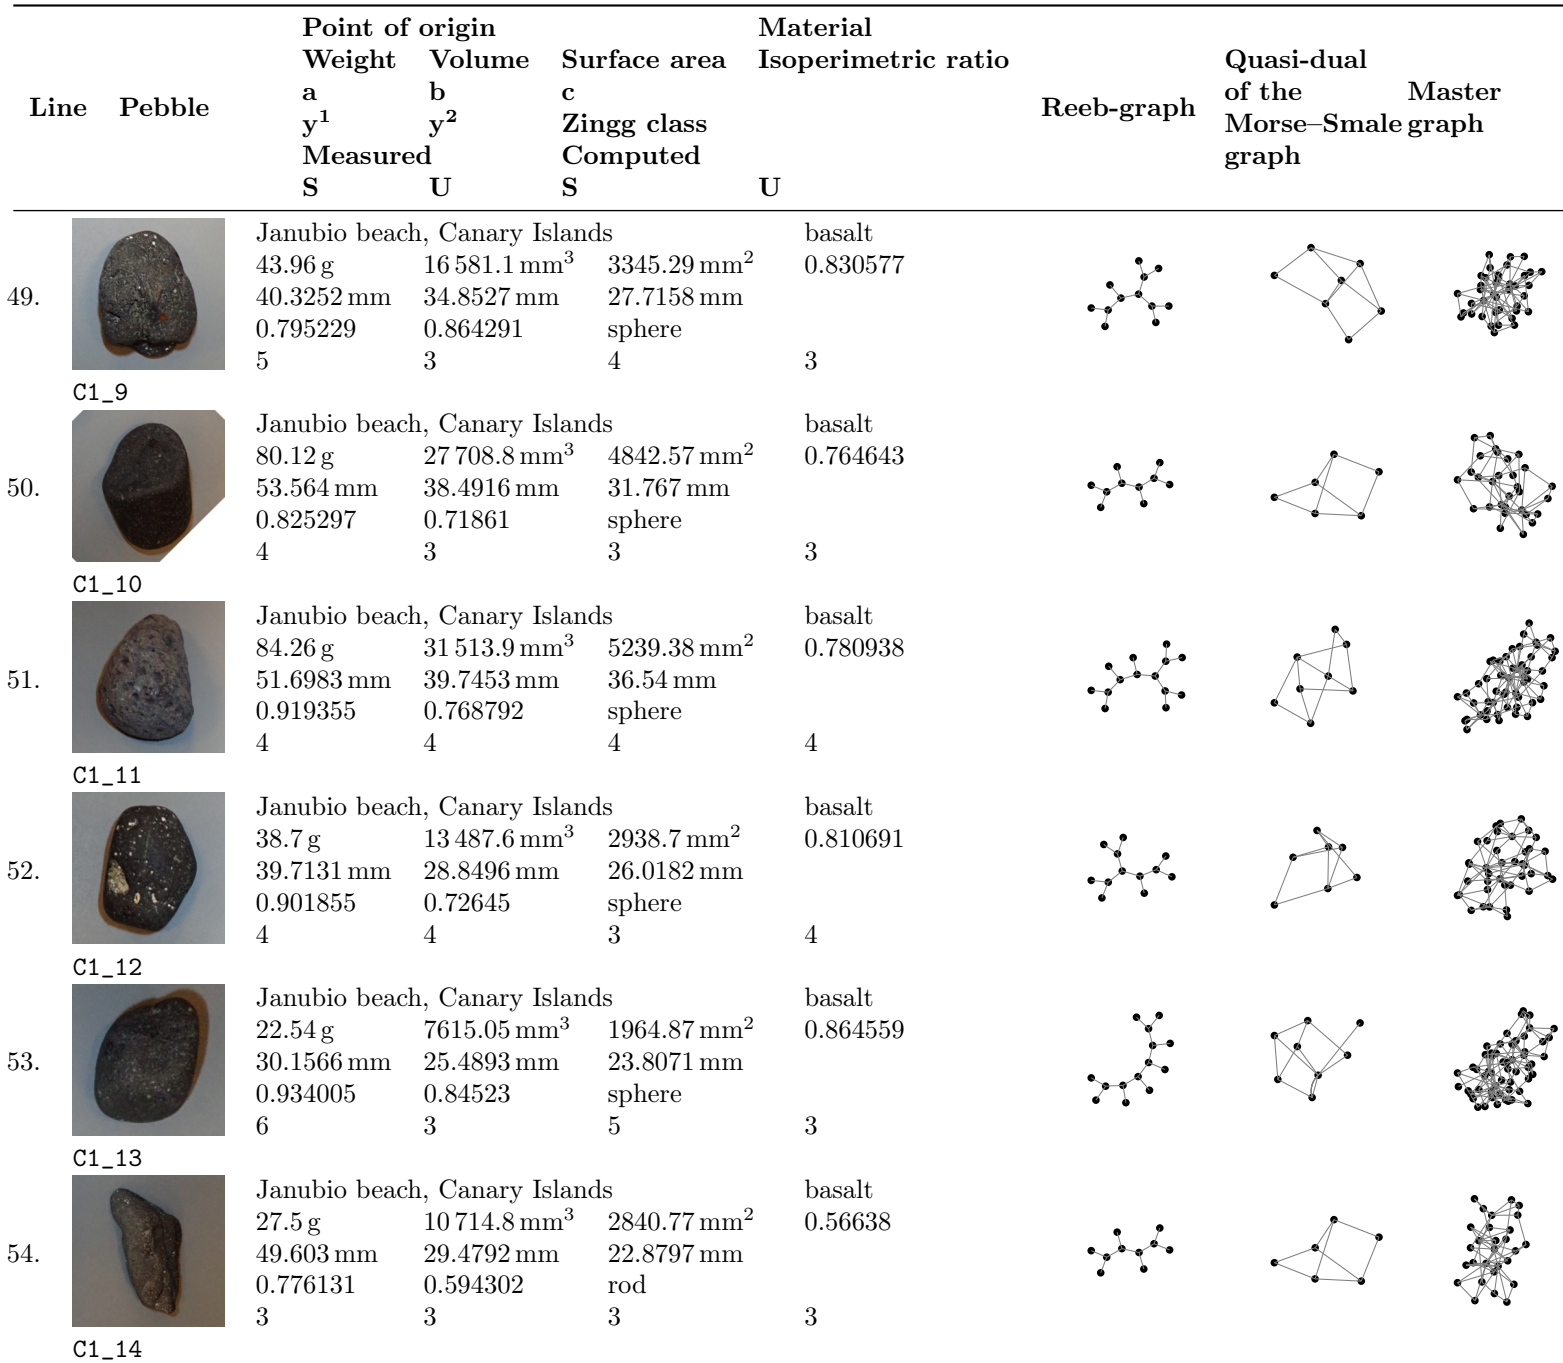   | 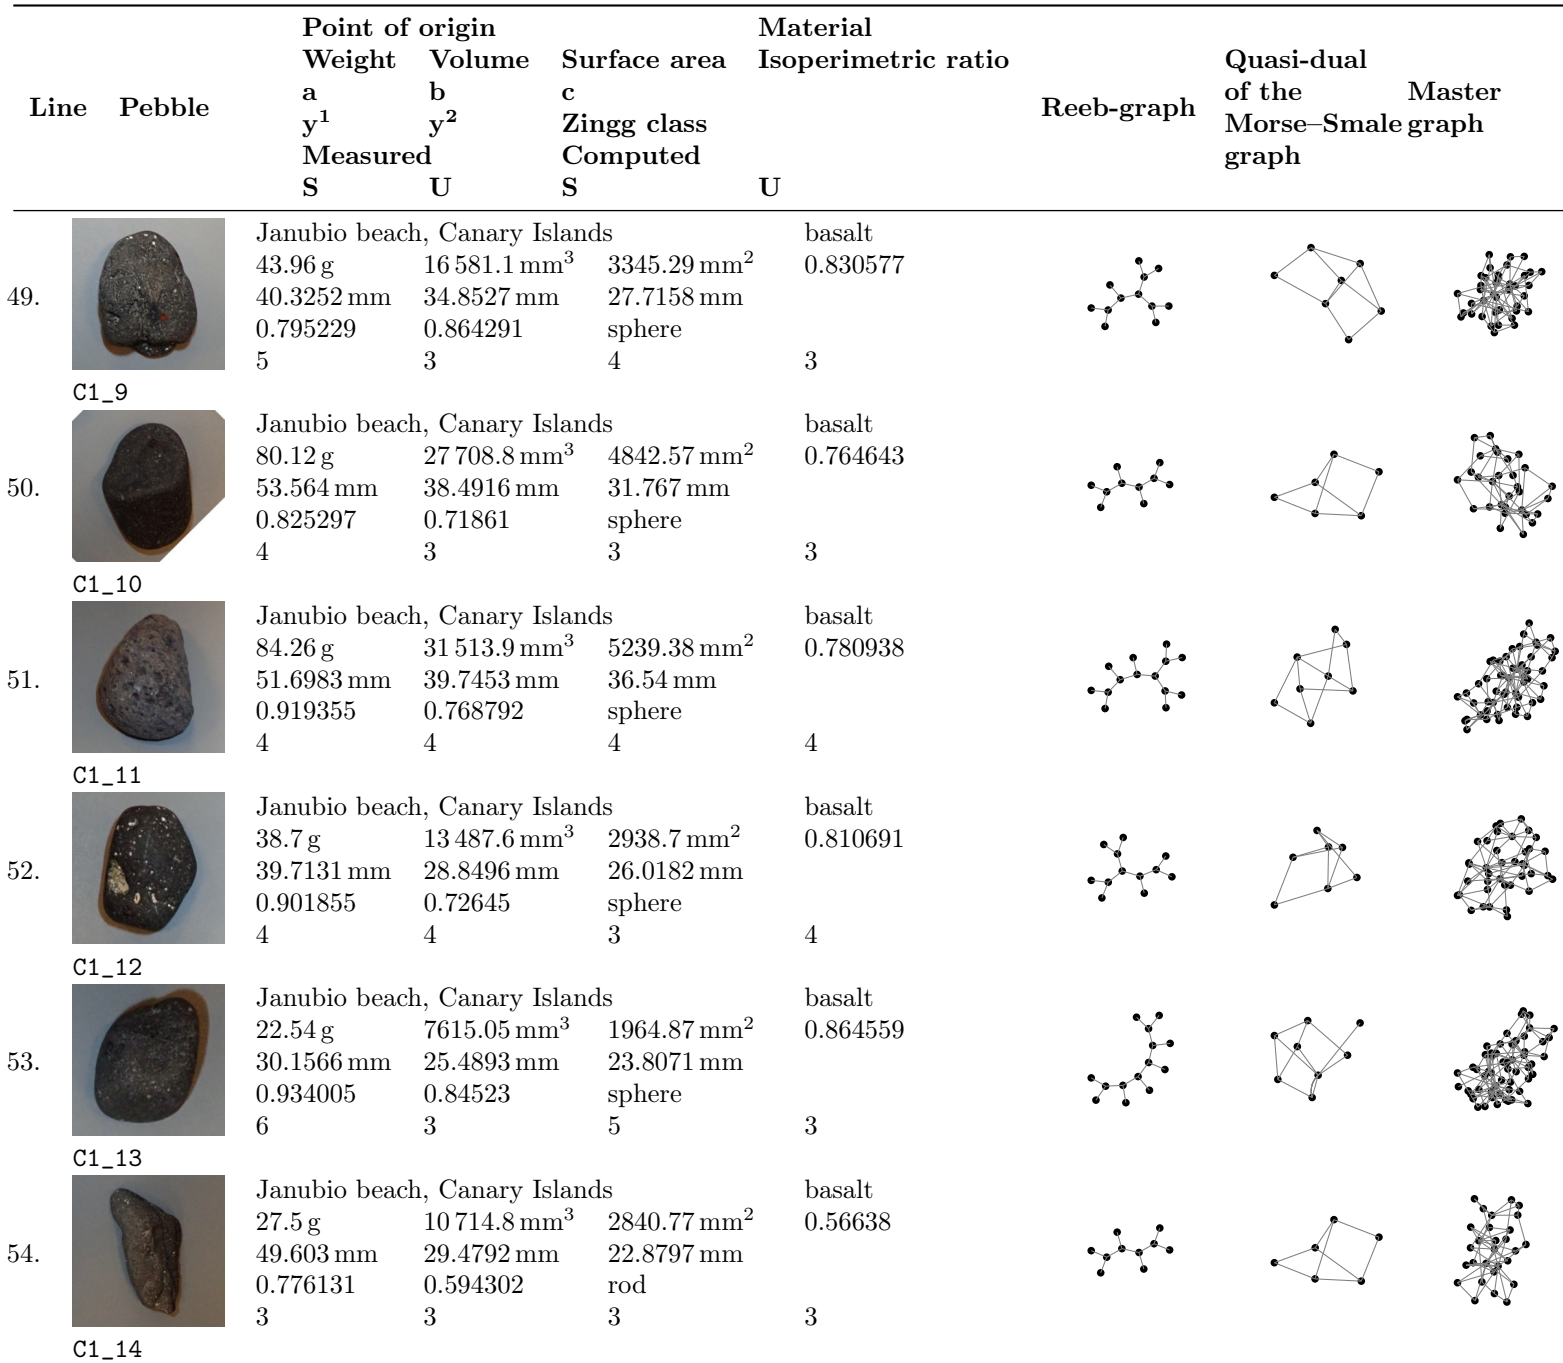   | 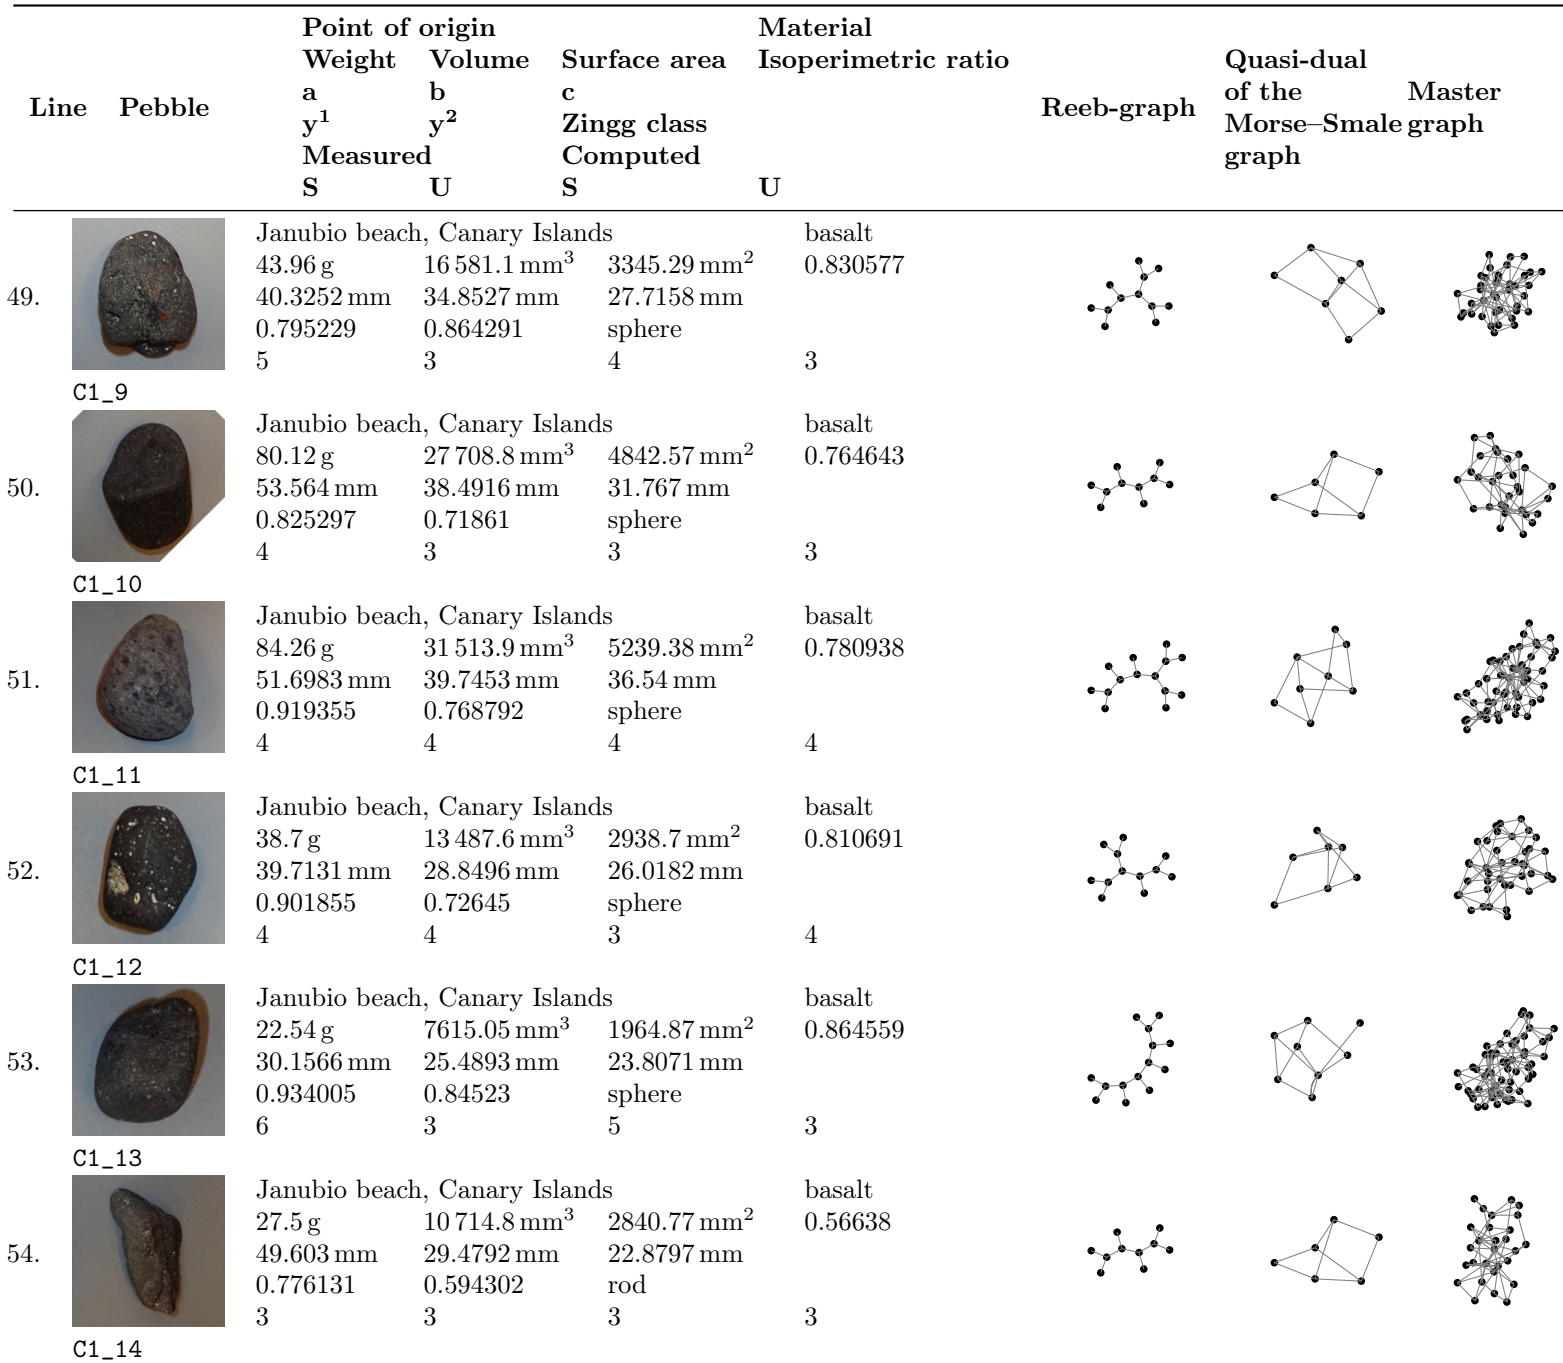   |
|      | C1_9                                                                                | 43.96 g                              | 16 581.1 mm <sup>3</sup> |                                                      |                                      |                                                                                       |                                                                                       |                                                                                       |
|      |                                                                                     | 40.3252 mm                           | 34.8527 mm               |                                                      |                                      |                                                                                       |                                                                                       |                                                                                       |
|      |                                                                                     | 0.795229                             | 0.864291                 |                                                      |                                      |                                                                                       |                                                                                       |                                                                                       |
|      |                                                                                     | 5                                    | 3                        |                                                      |                                      |                                                                                       |                                                                                       |                                                                                       |
| 50.  | 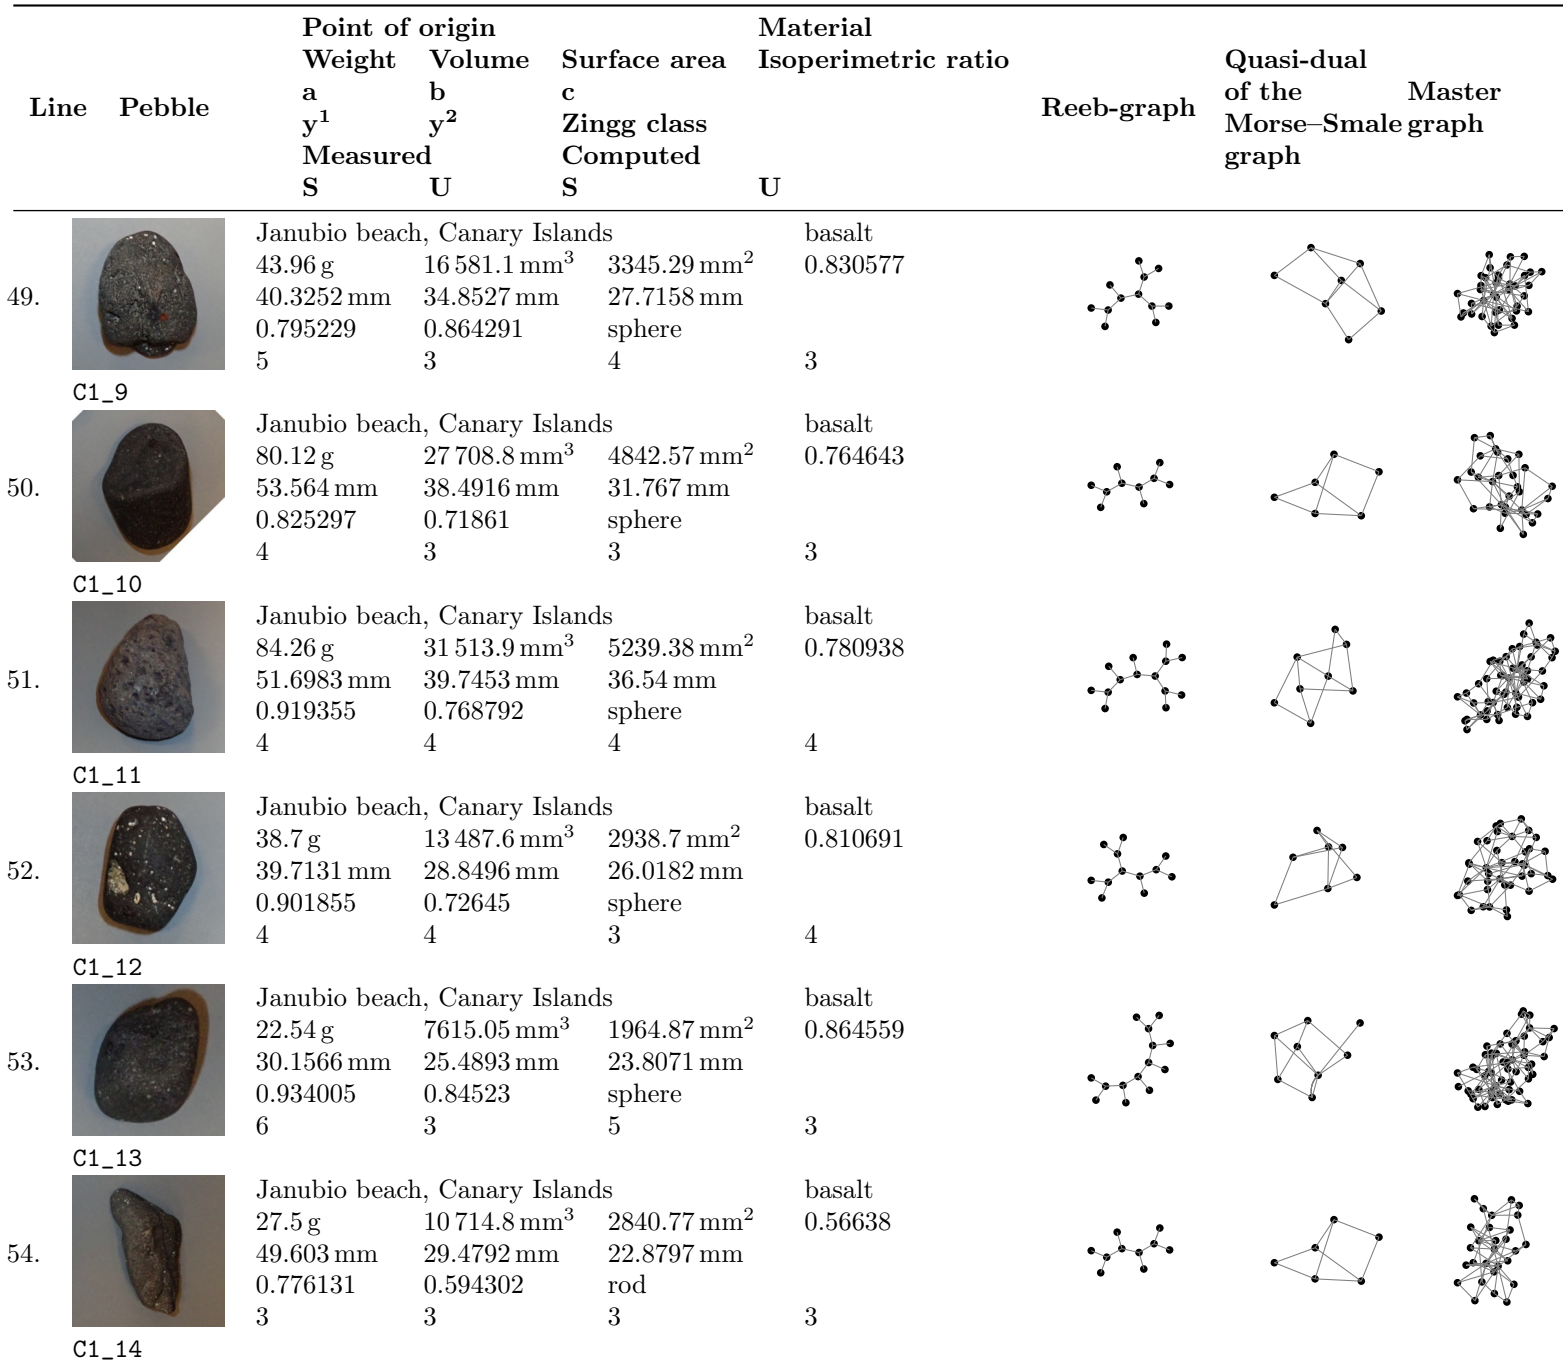   | Janubio beach, Canary Islands        |                          | 4842.57 mm <sup>2</sup><br>31.767 mm<br>sphere<br>3  | basalt<br>0.764643<br><br>3          | 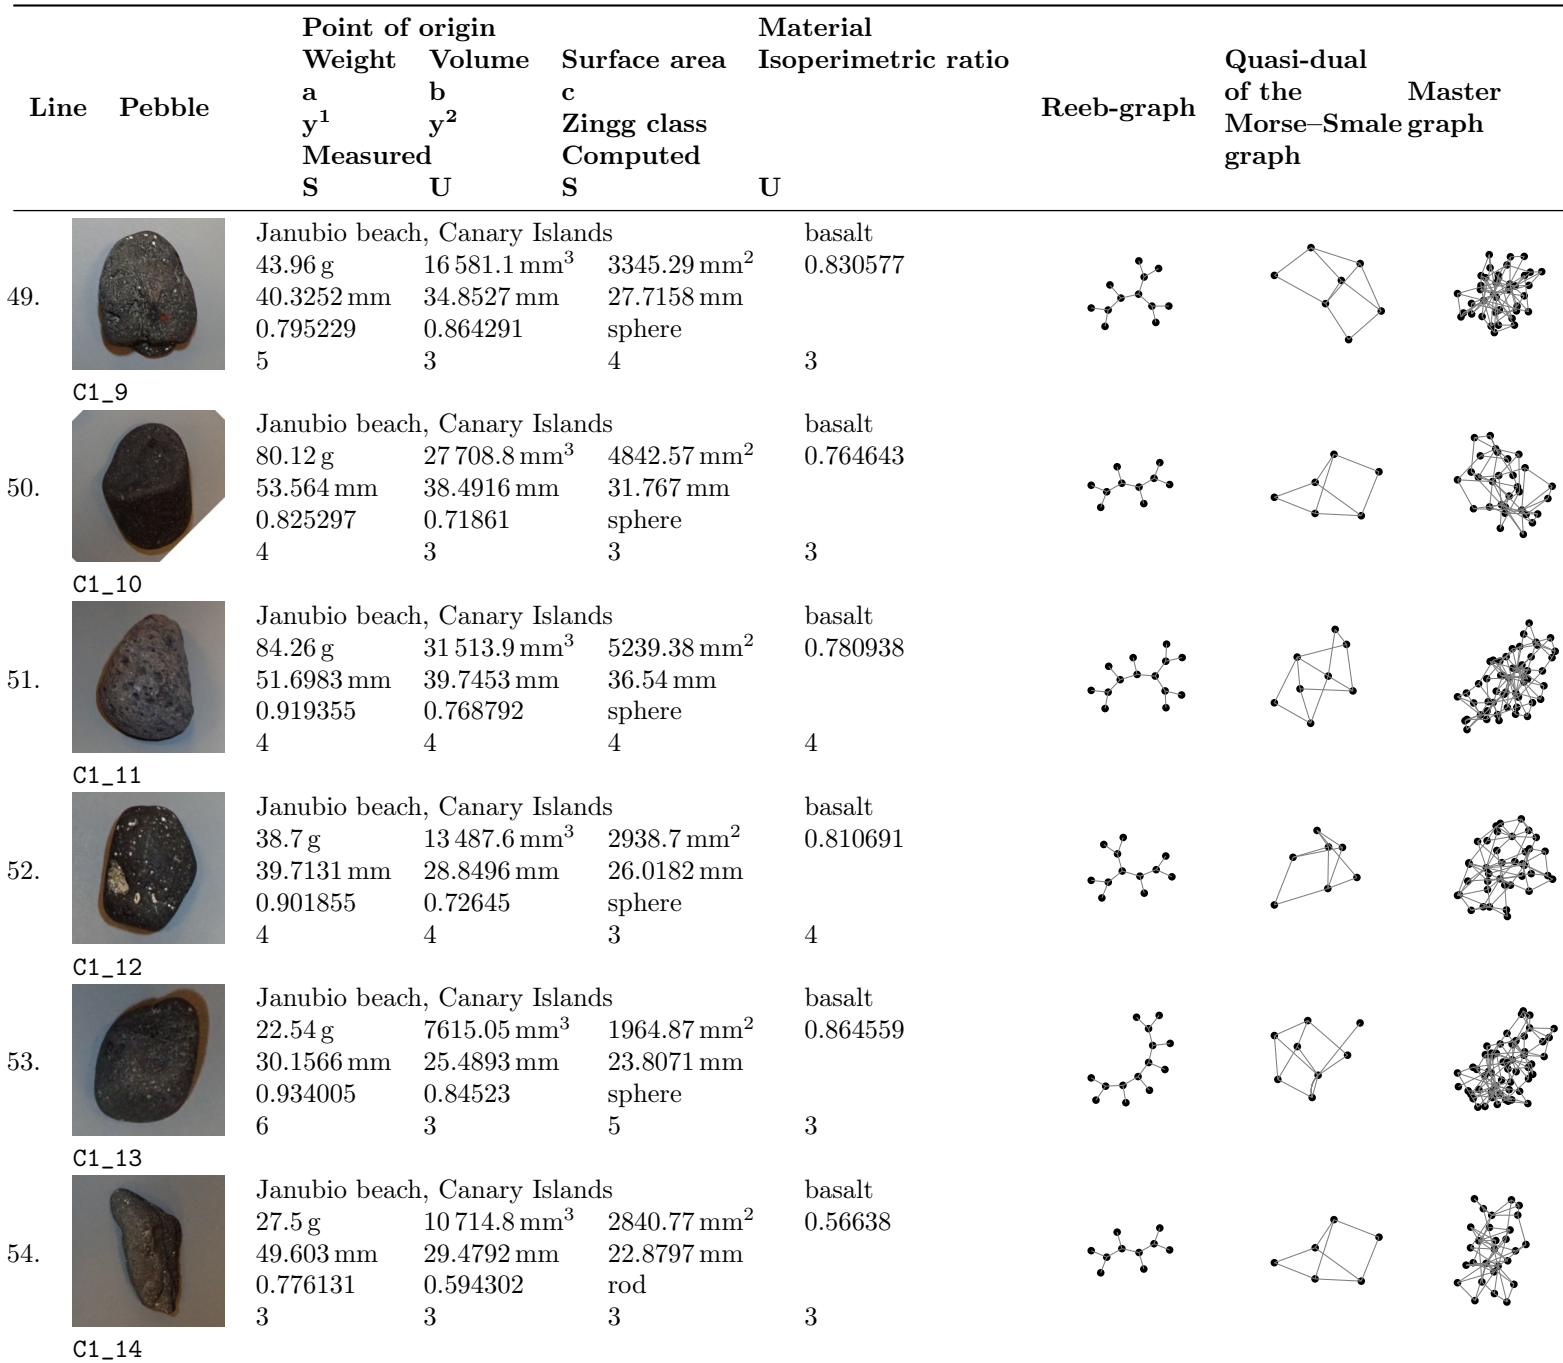   | 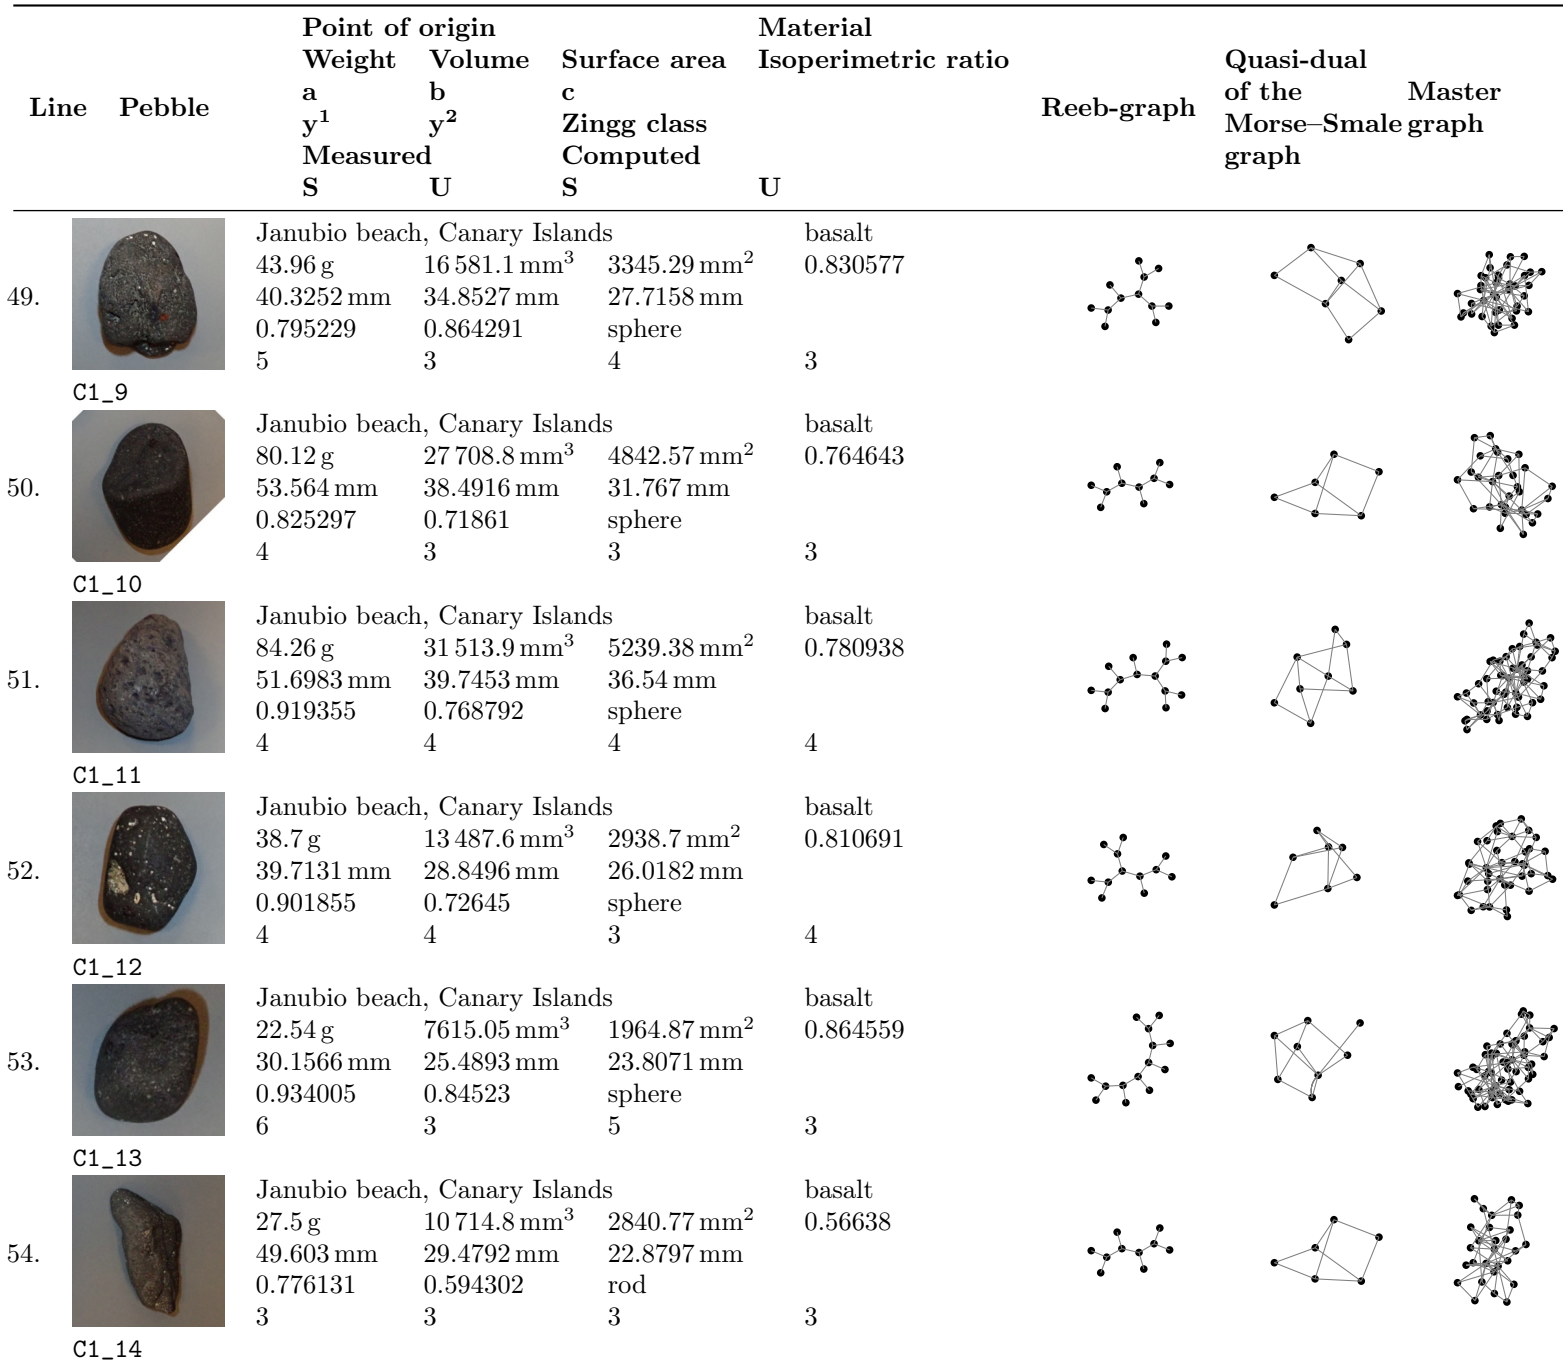   | 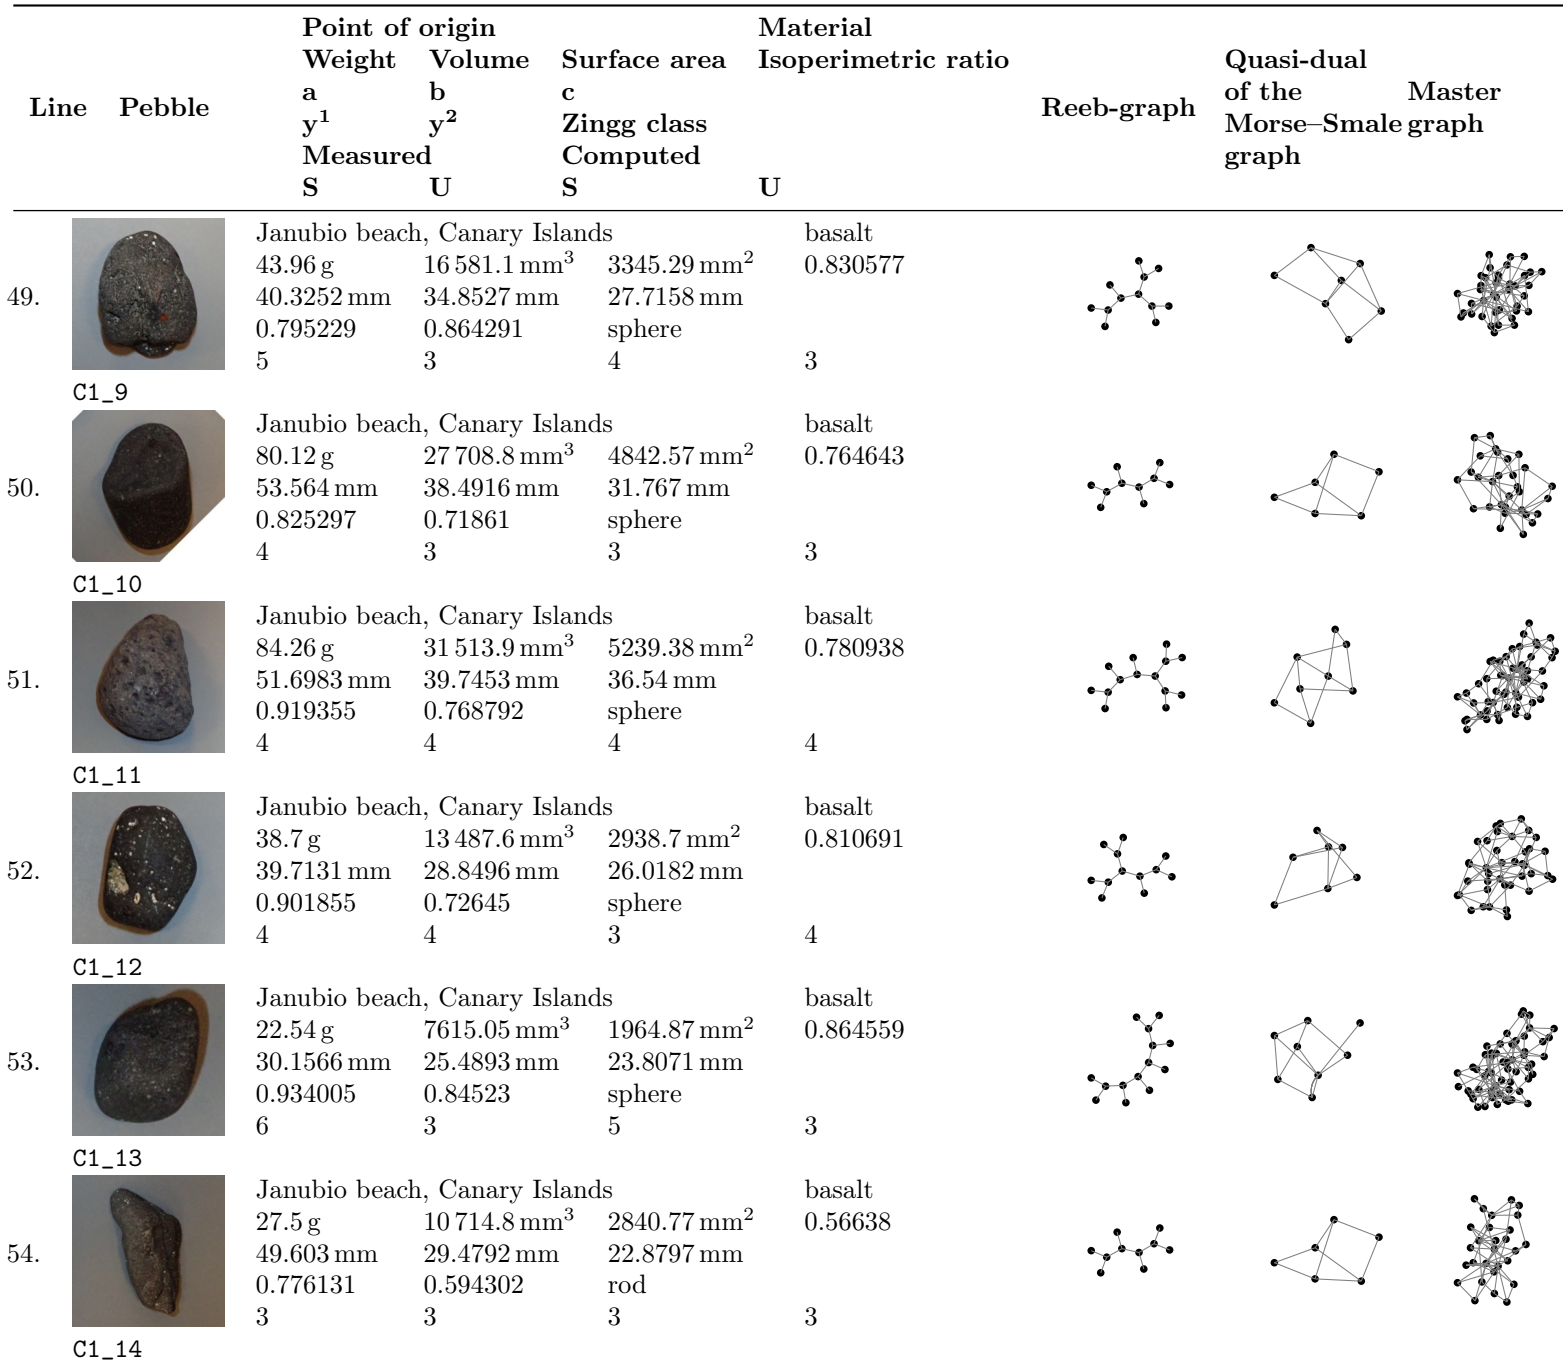   |
|      | C1_10                                                                               | 80.12 g                              | 27 708.8 mm <sup>3</sup> |                                                      |                                      |                                                                                       |                                                                                       |                                                                                       |
|      |                                                                                     | 53.564 mm                            | 38.4916 mm               |                                                      |                                      |                                                                                       |                                                                                       |                                                                                       |
|      |                                                                                     | 0.825297                             | 0.71861                  |                                                      |                                      |                                                                                       |                                                                                       |                                                                                       |
|      |                                                                                     | 4                                    | 3                        |                                                      |                                      |                                                                                       |                                                                                       |                                                                                       |
| 51.  | 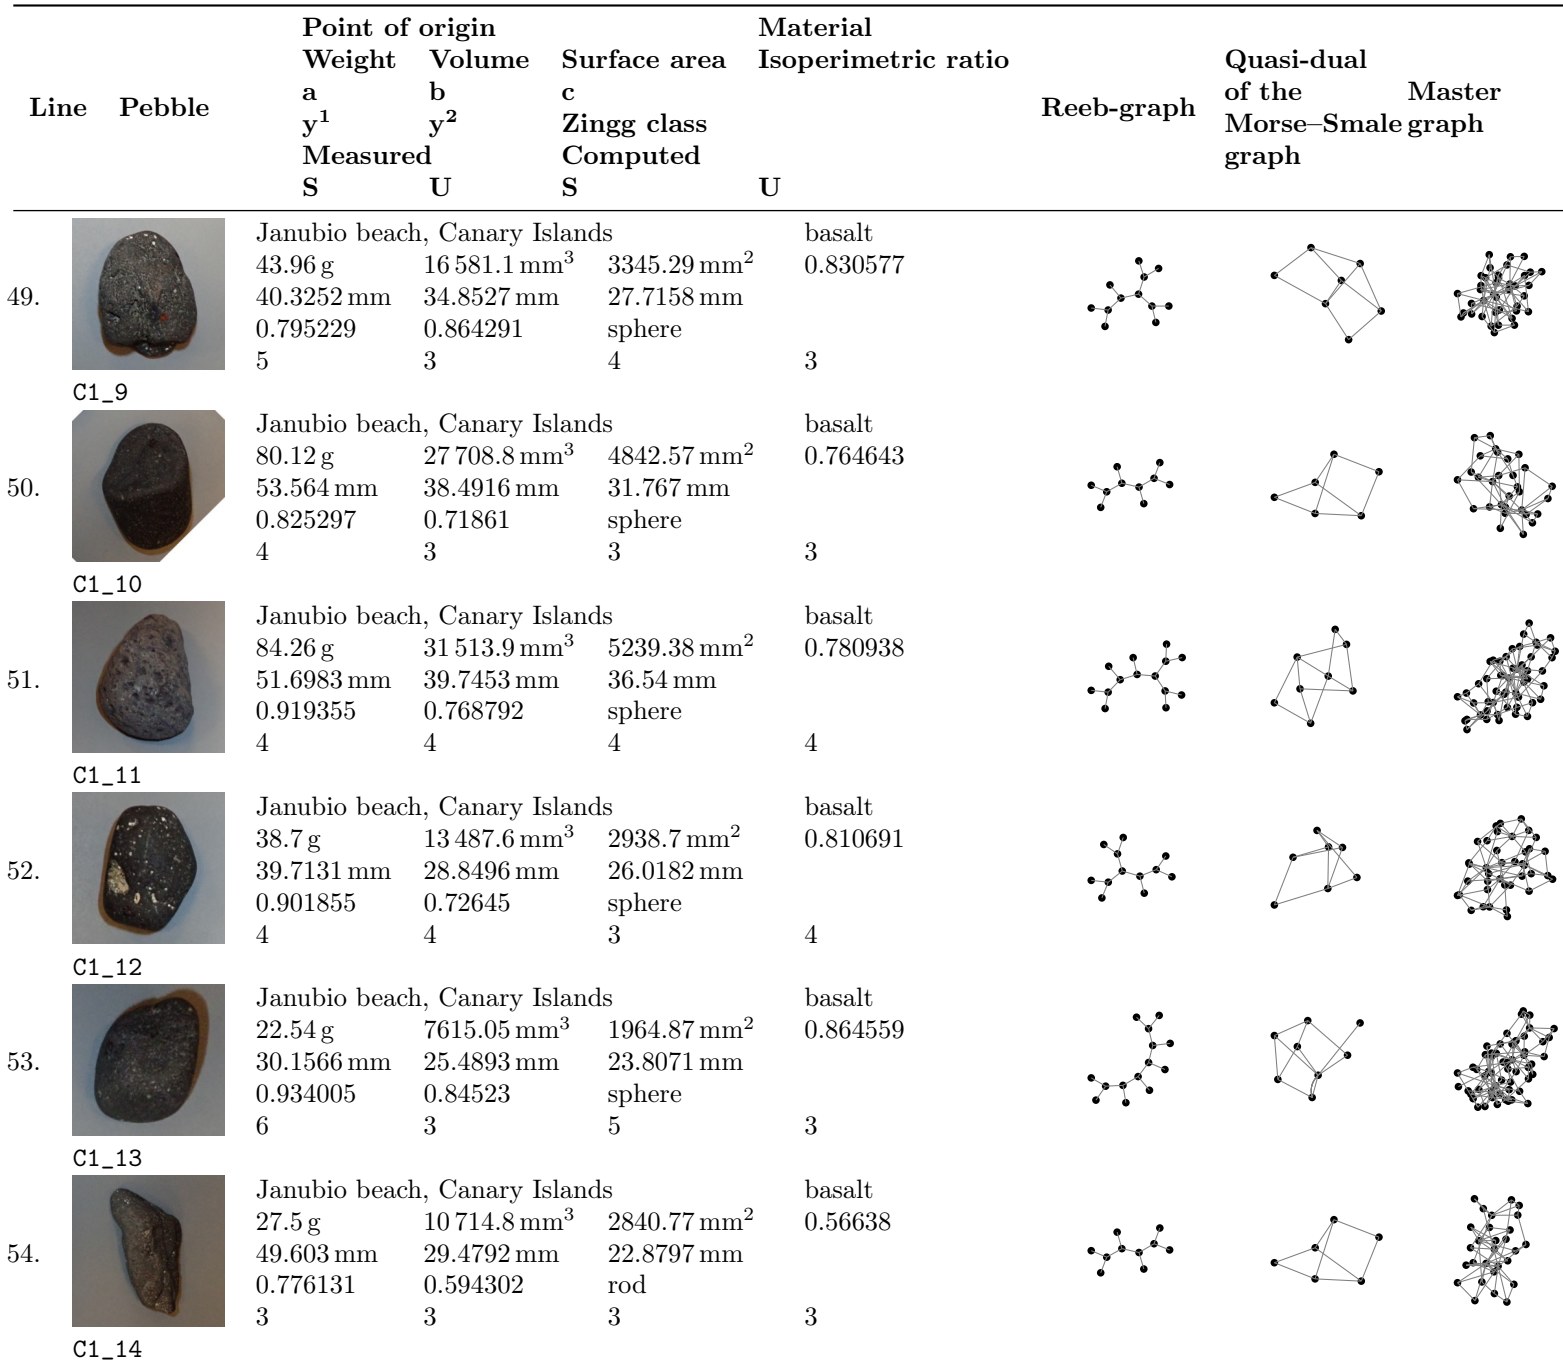   | Janubio beach, Canary Islands        |                          | 5239.38 mm <sup>2</sup><br>36.54 mm<br>sphere<br>4   | basalt<br>0.780938<br><br>4          | 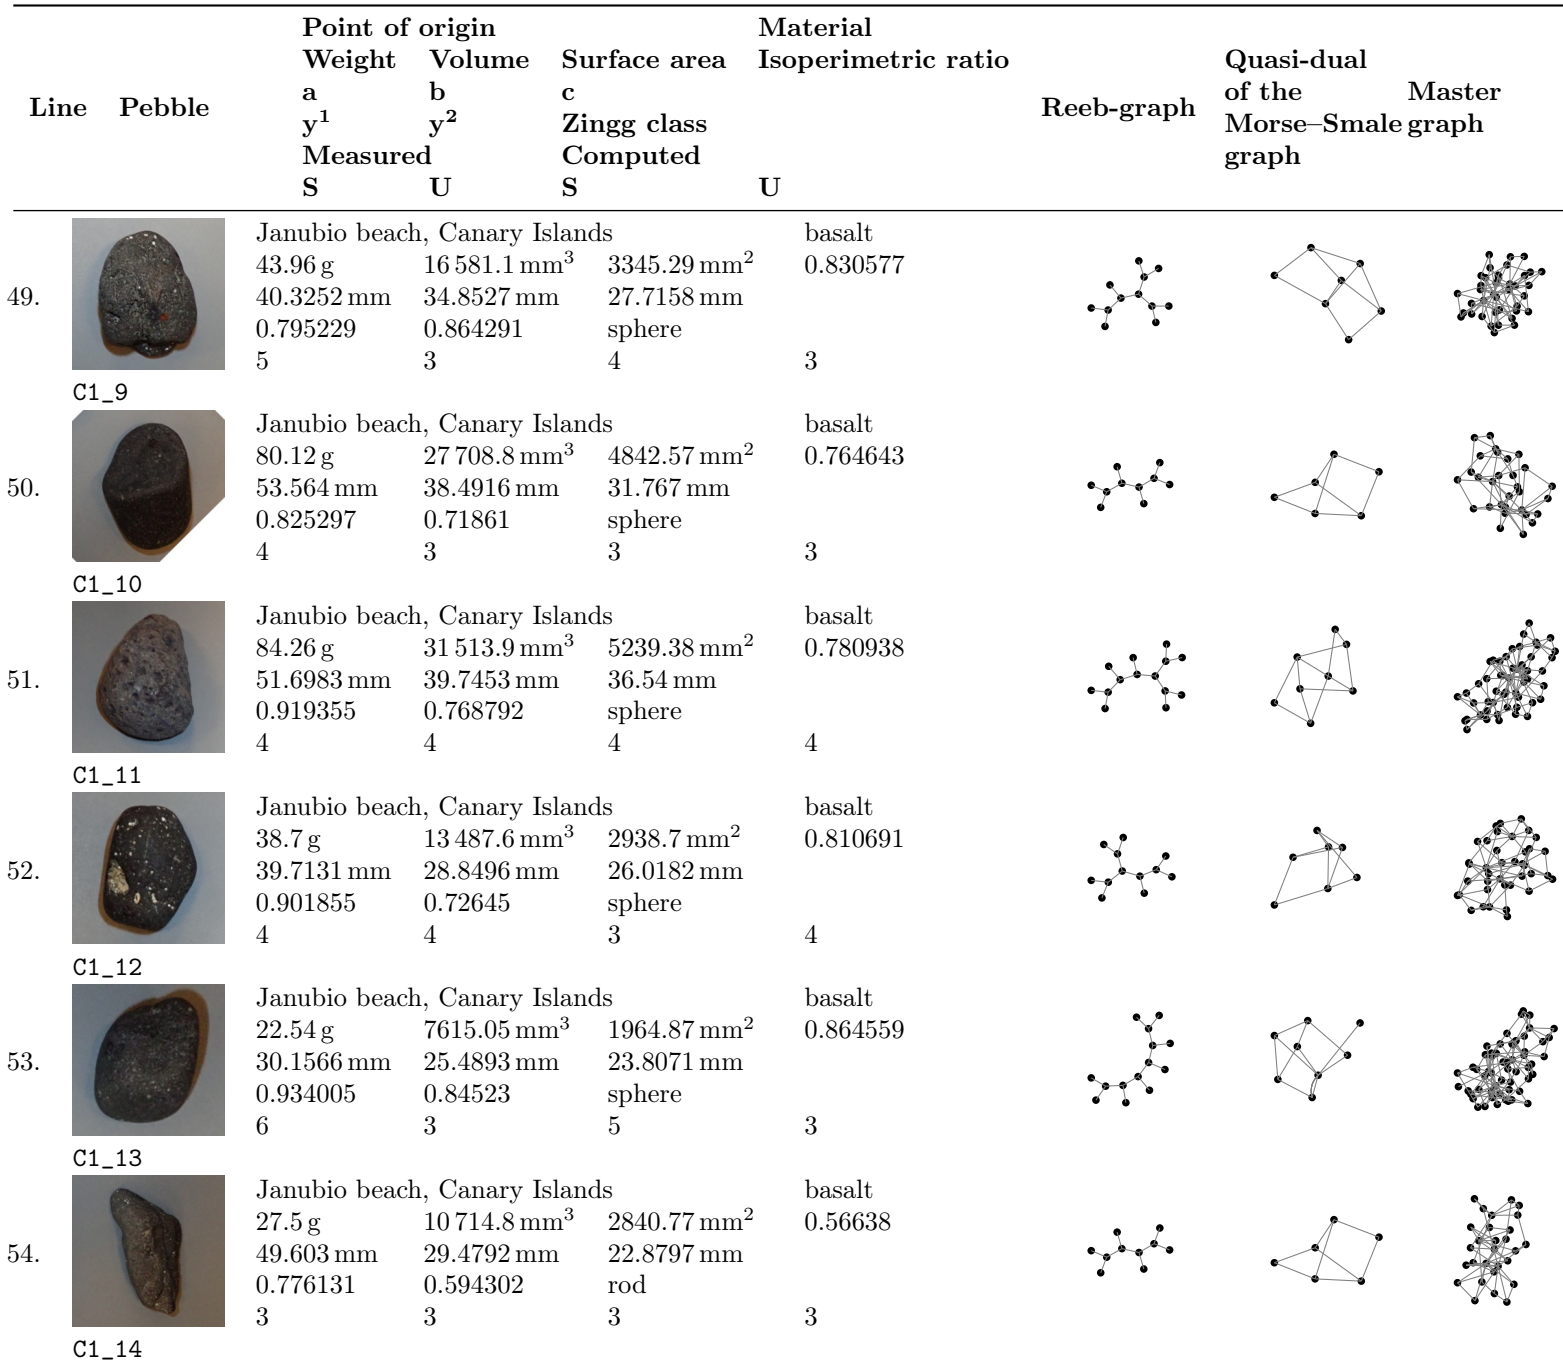   | 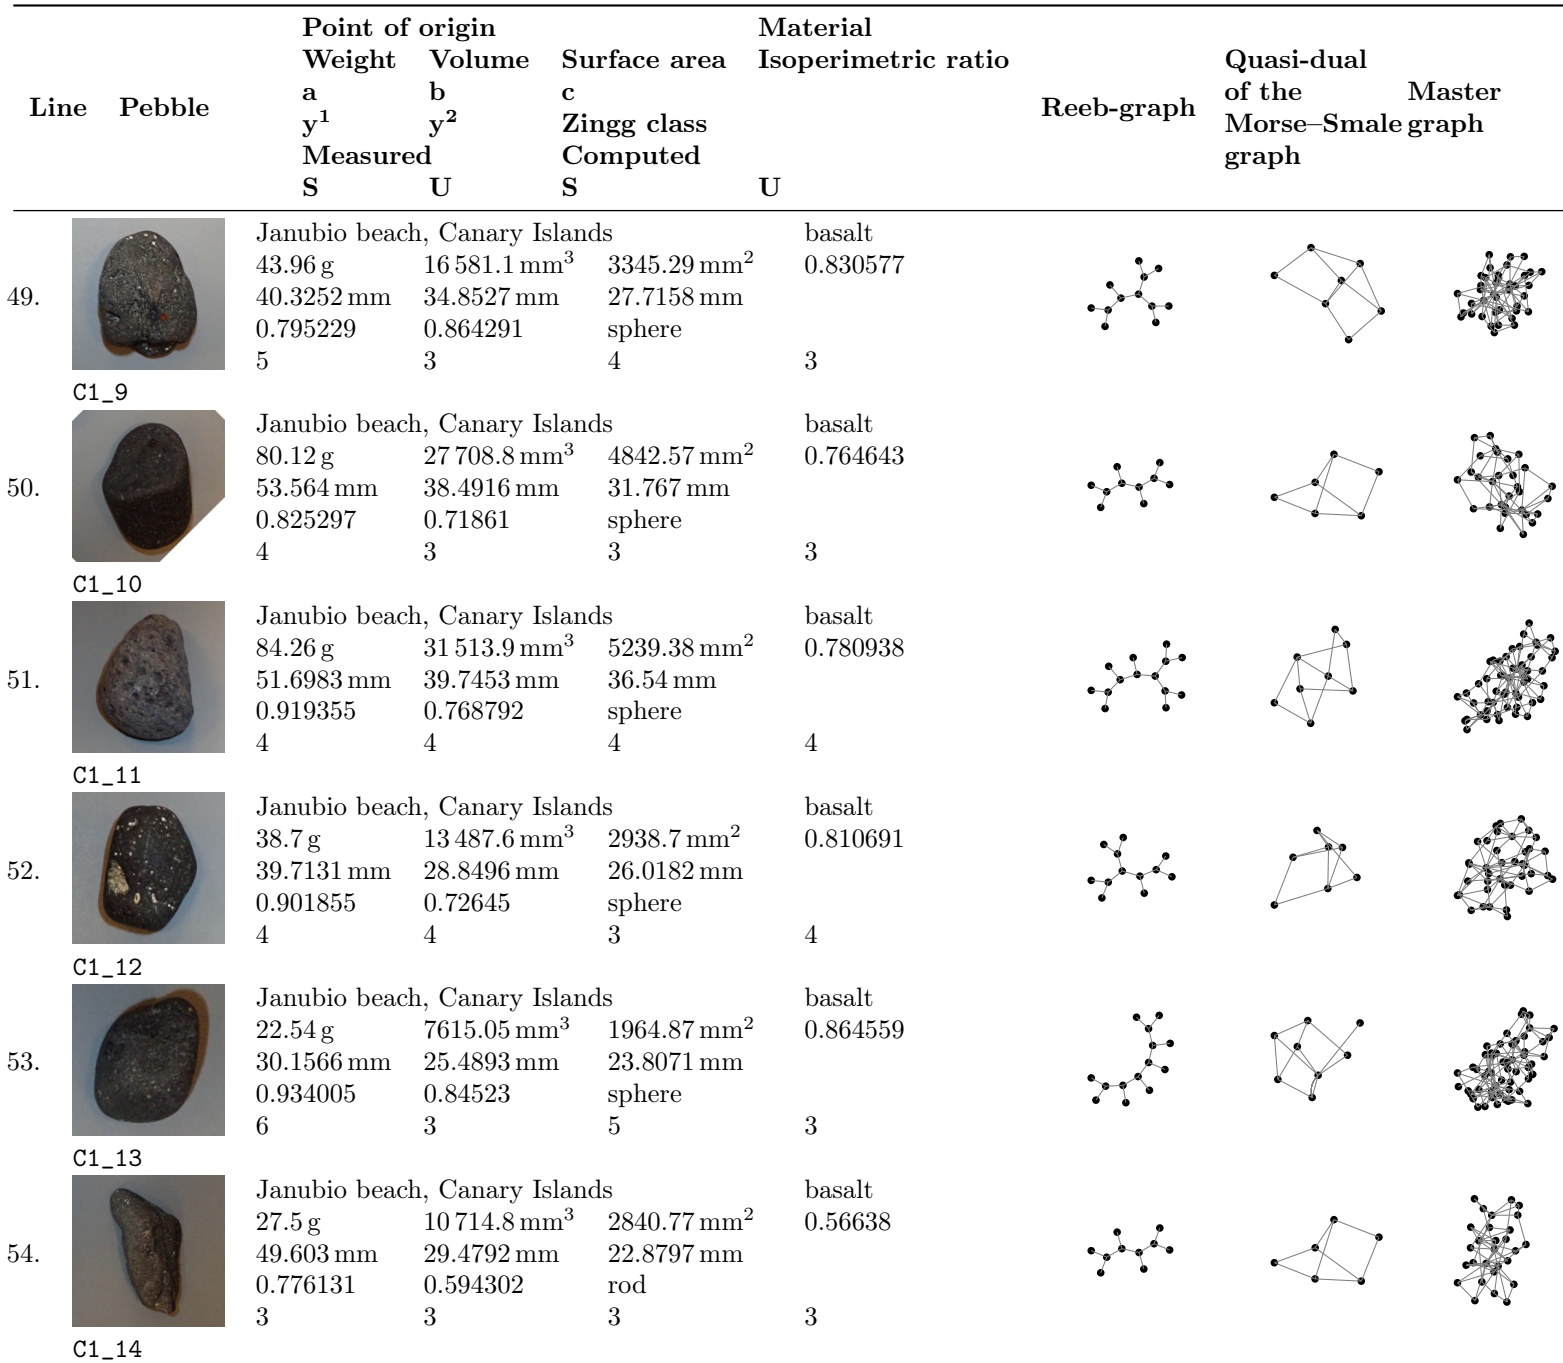   | 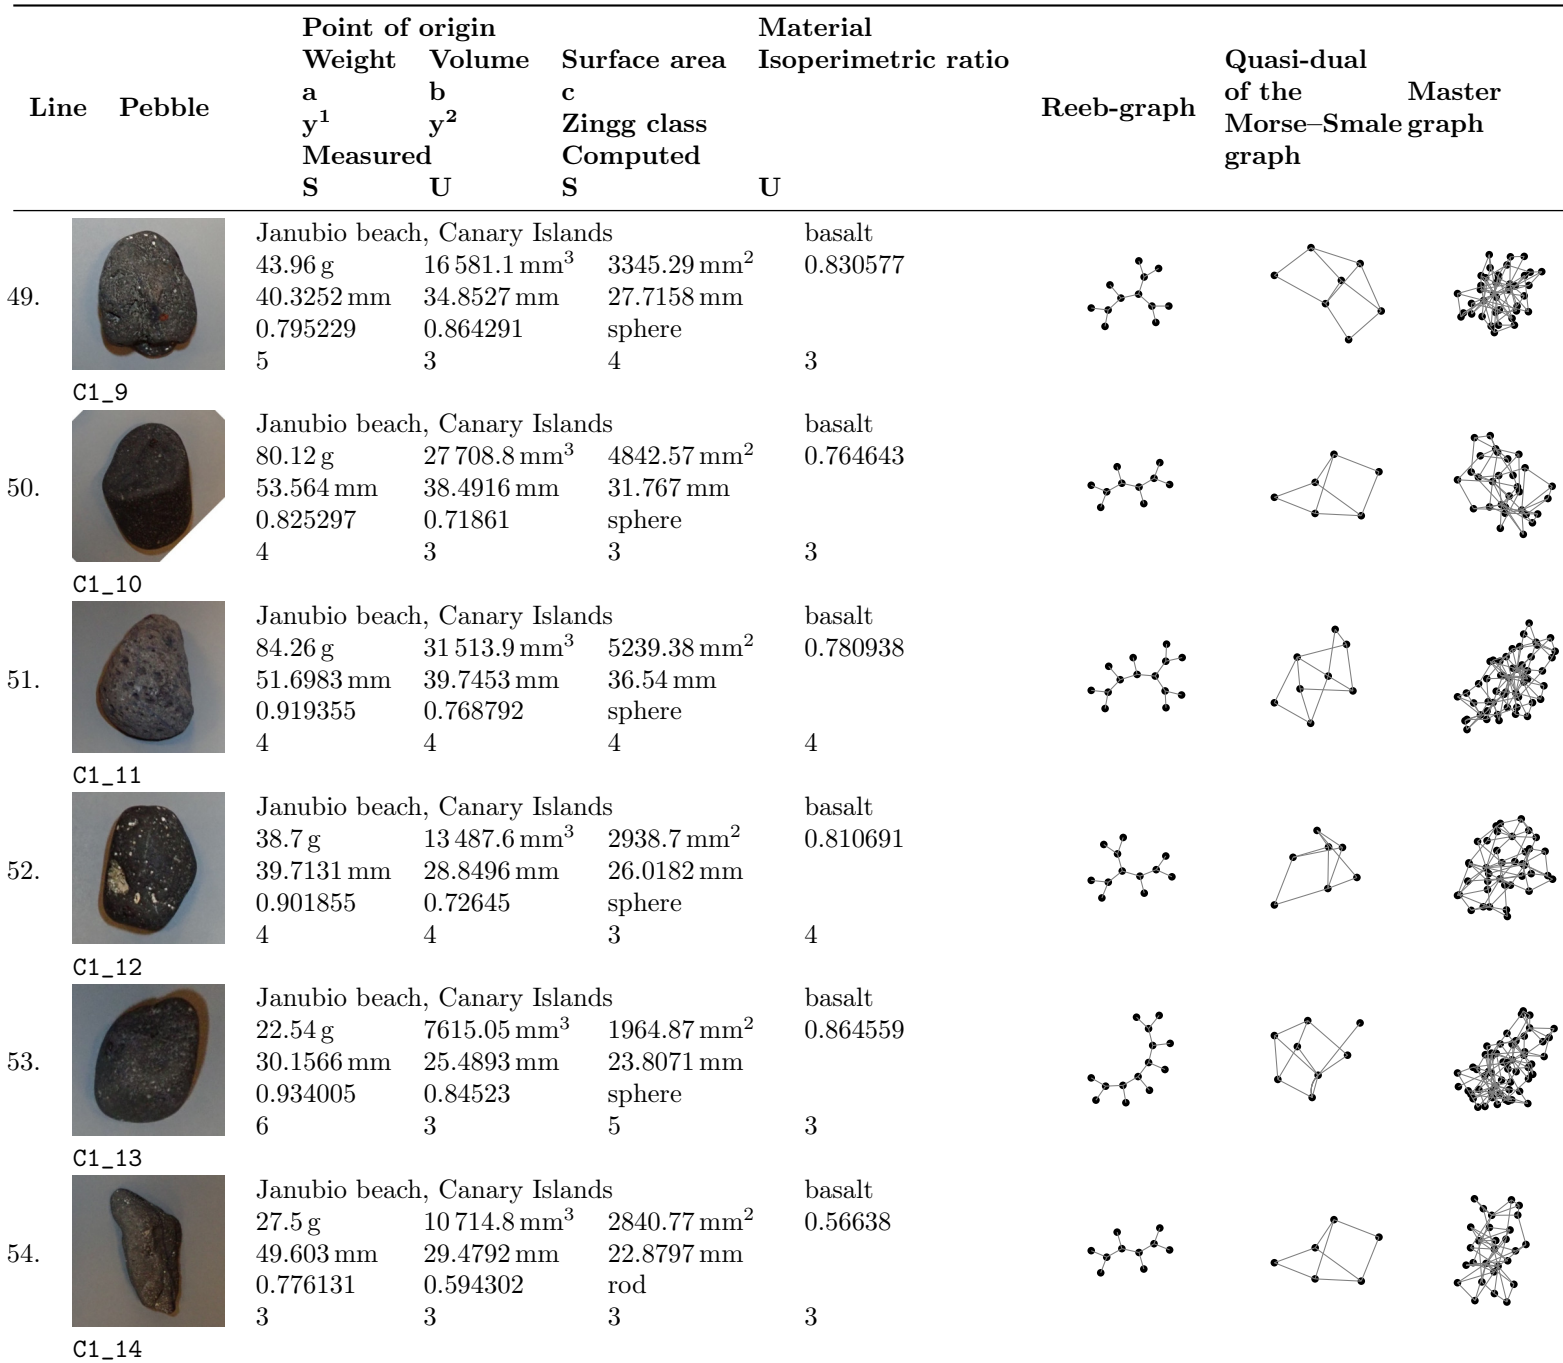   |
|      | C1_11                                                                               | 84.26 g                              | 31 513.9 mm <sup>3</sup> |                                                      |                                      |                                                                                       |                                                                                       |                                                                                       |
|      |                                                                                     | 51.6983 mm                           | 39.7453 mm               |                                                      |                                      |                                                                                       |                                                                                       |                                                                                       |
|      |                                                                                     | 0.919355                             | 0.768792                 |                                                      |                                      |                                                                                       |                                                                                       |                                                                                       |
|      |                                                                                     | 4                                    | 4                        |                                                      |                                      |                                                                                       |                                                                                       |                                                                                       |
| 52.  | 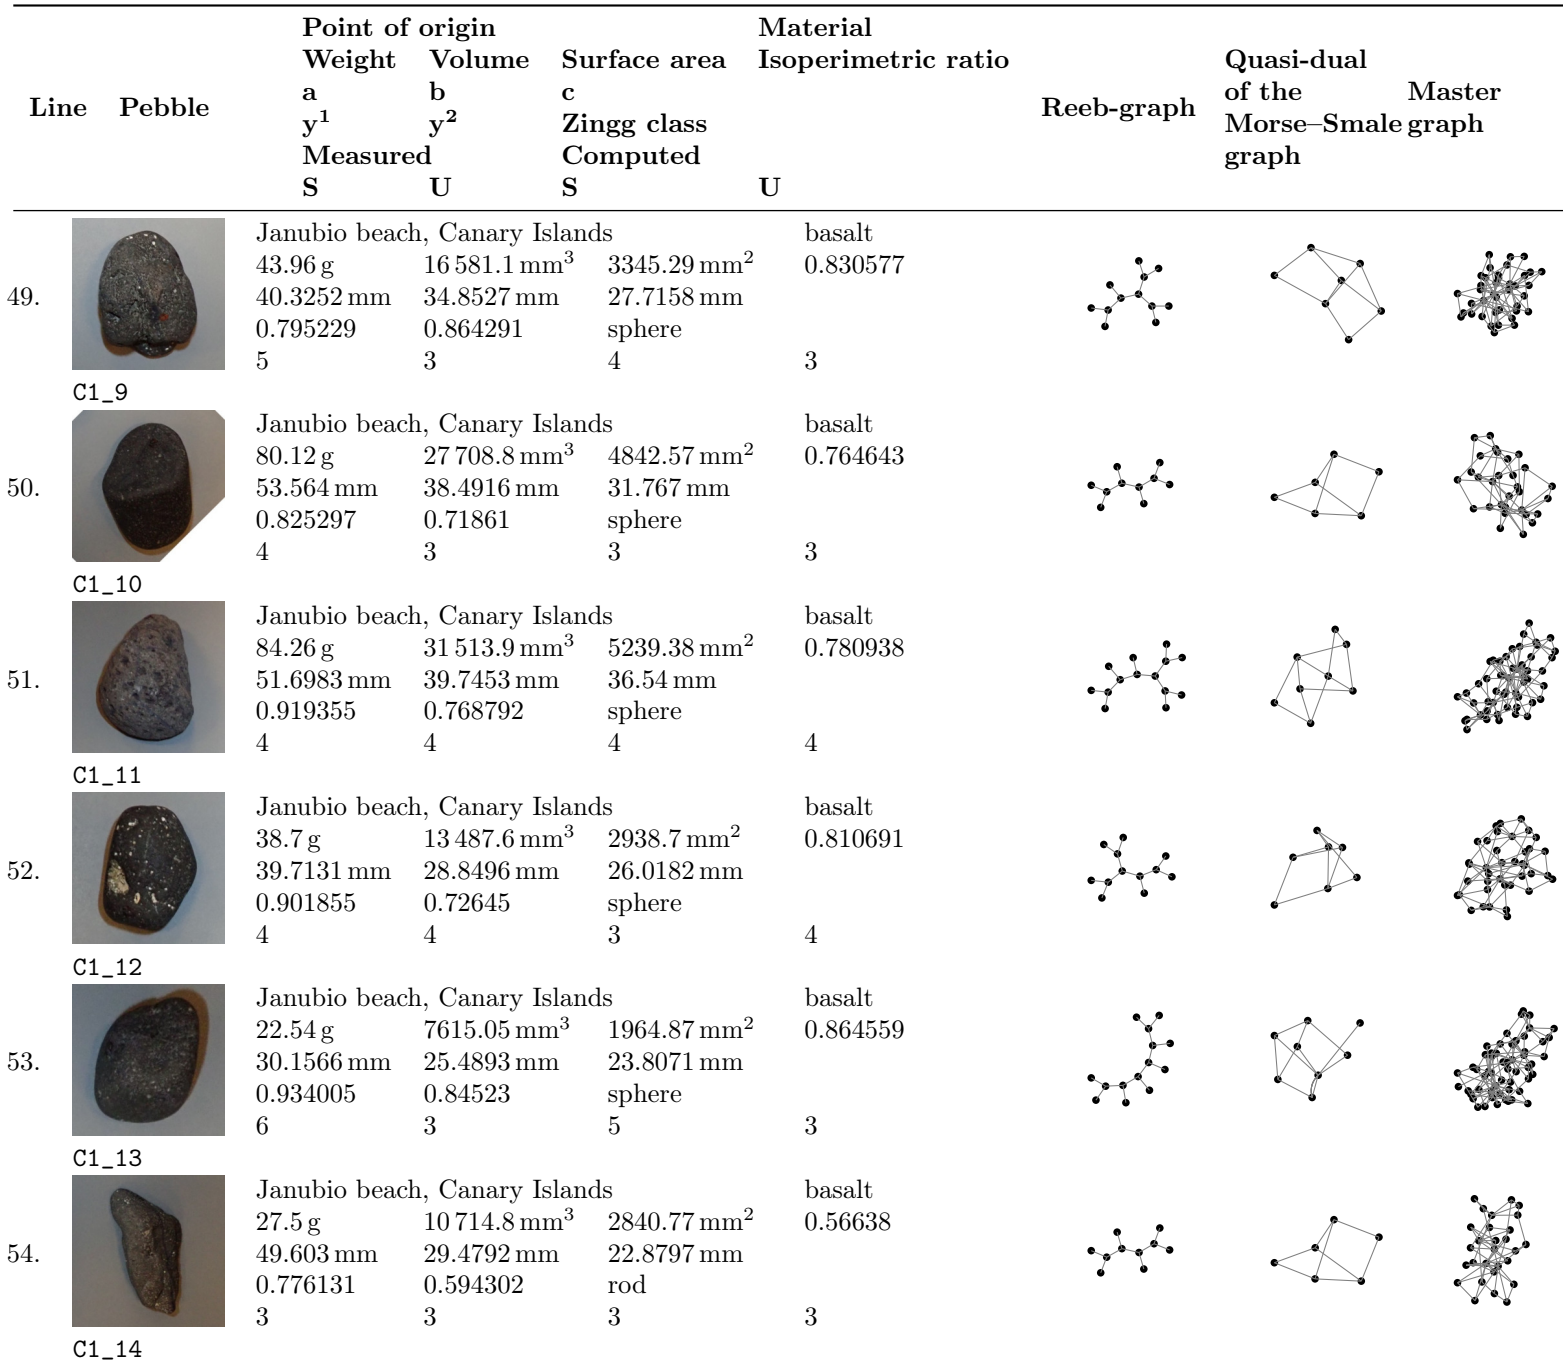  | Janubio beach, Canary Islands        |                          | 2938.7 mm <sup>2</sup><br>26.0182 mm<br>sphere<br>3  | basalt<br>0.810691<br><br>4          | 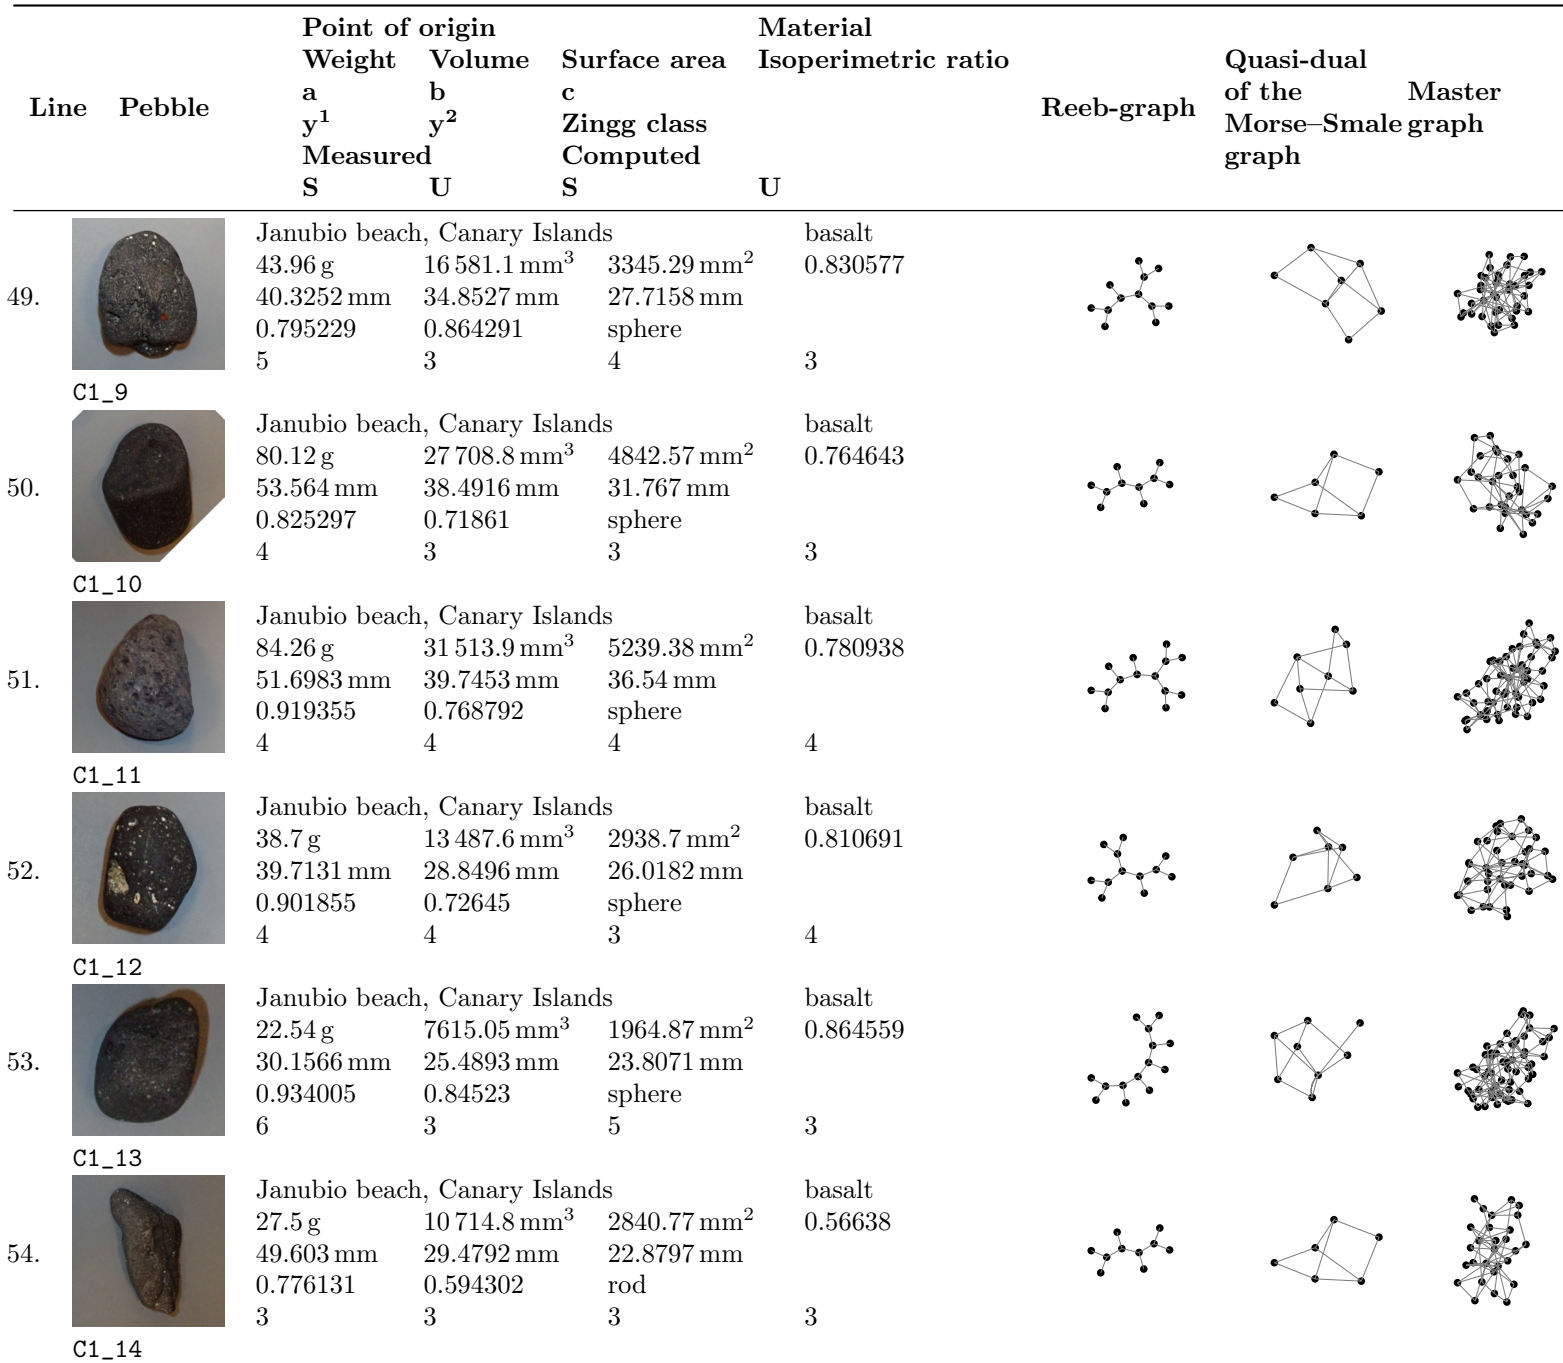  | 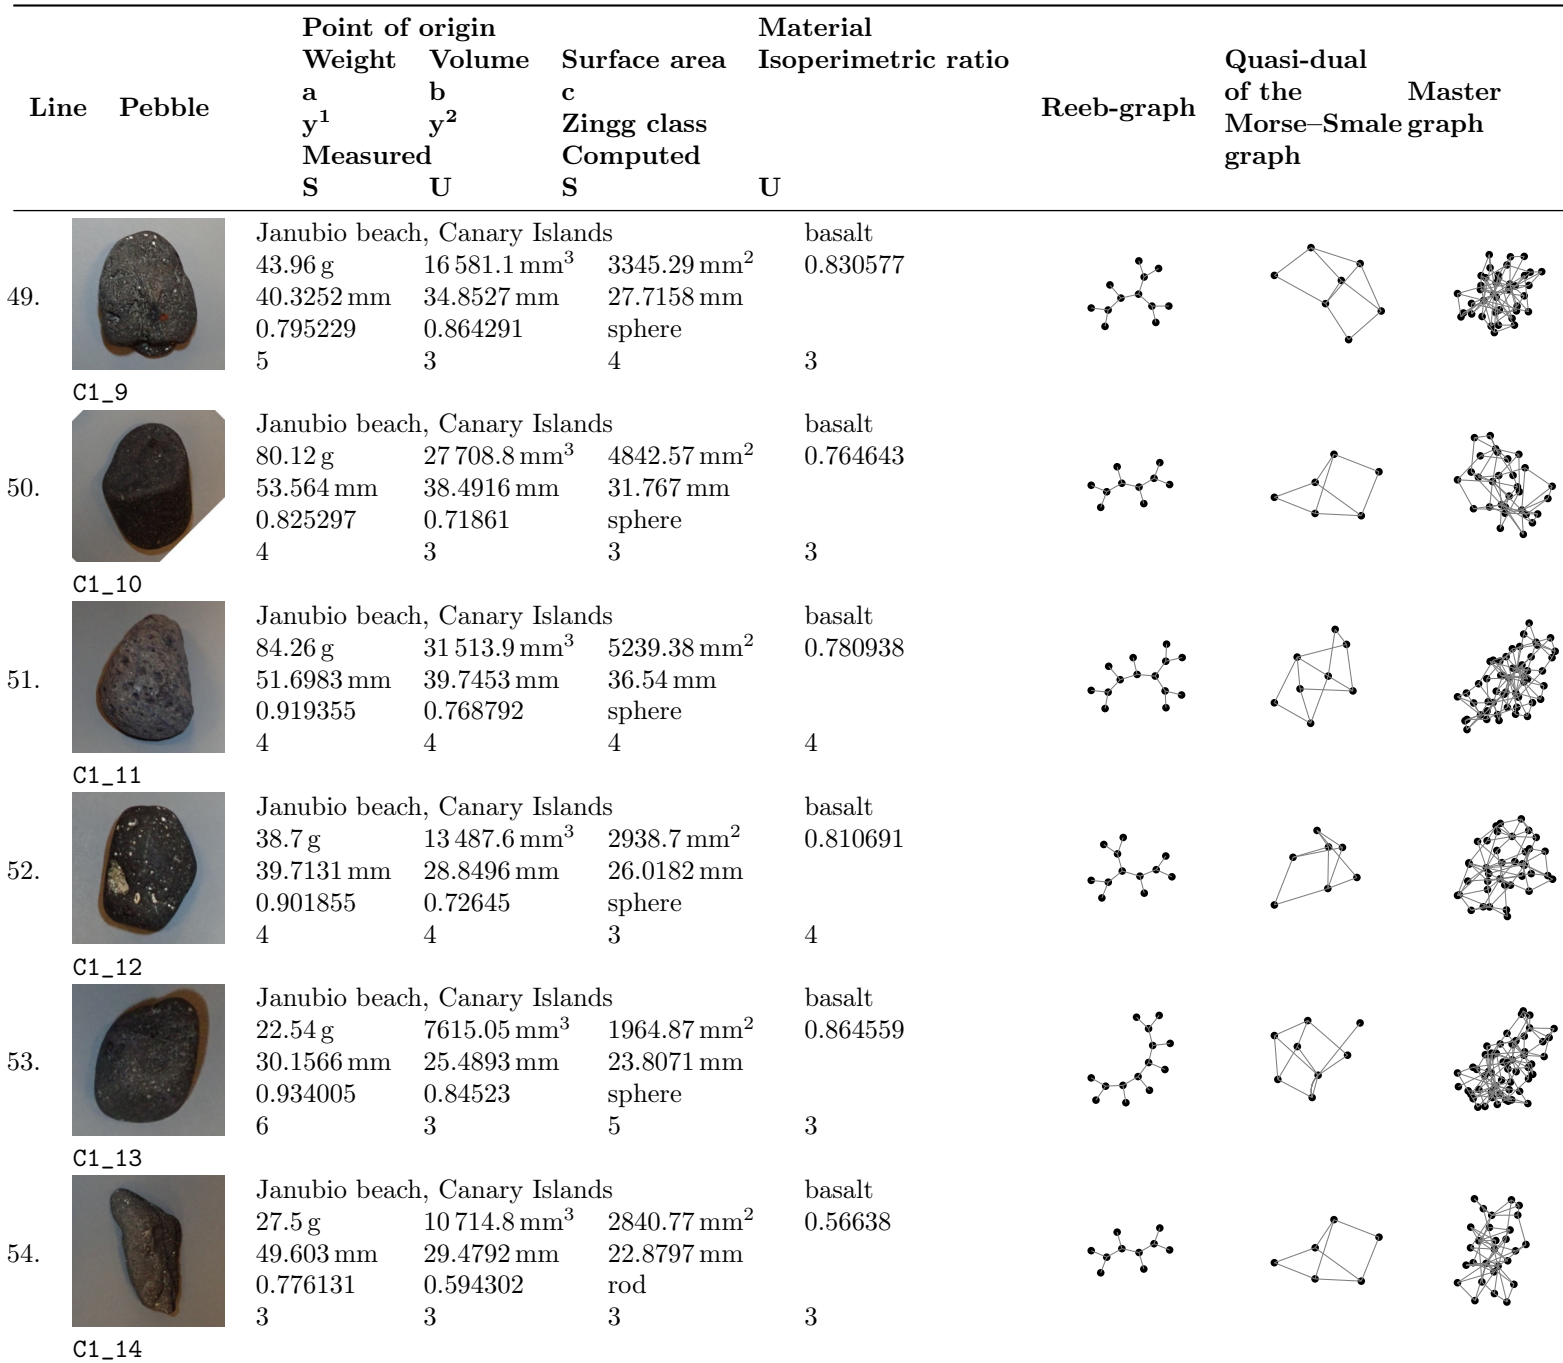  | 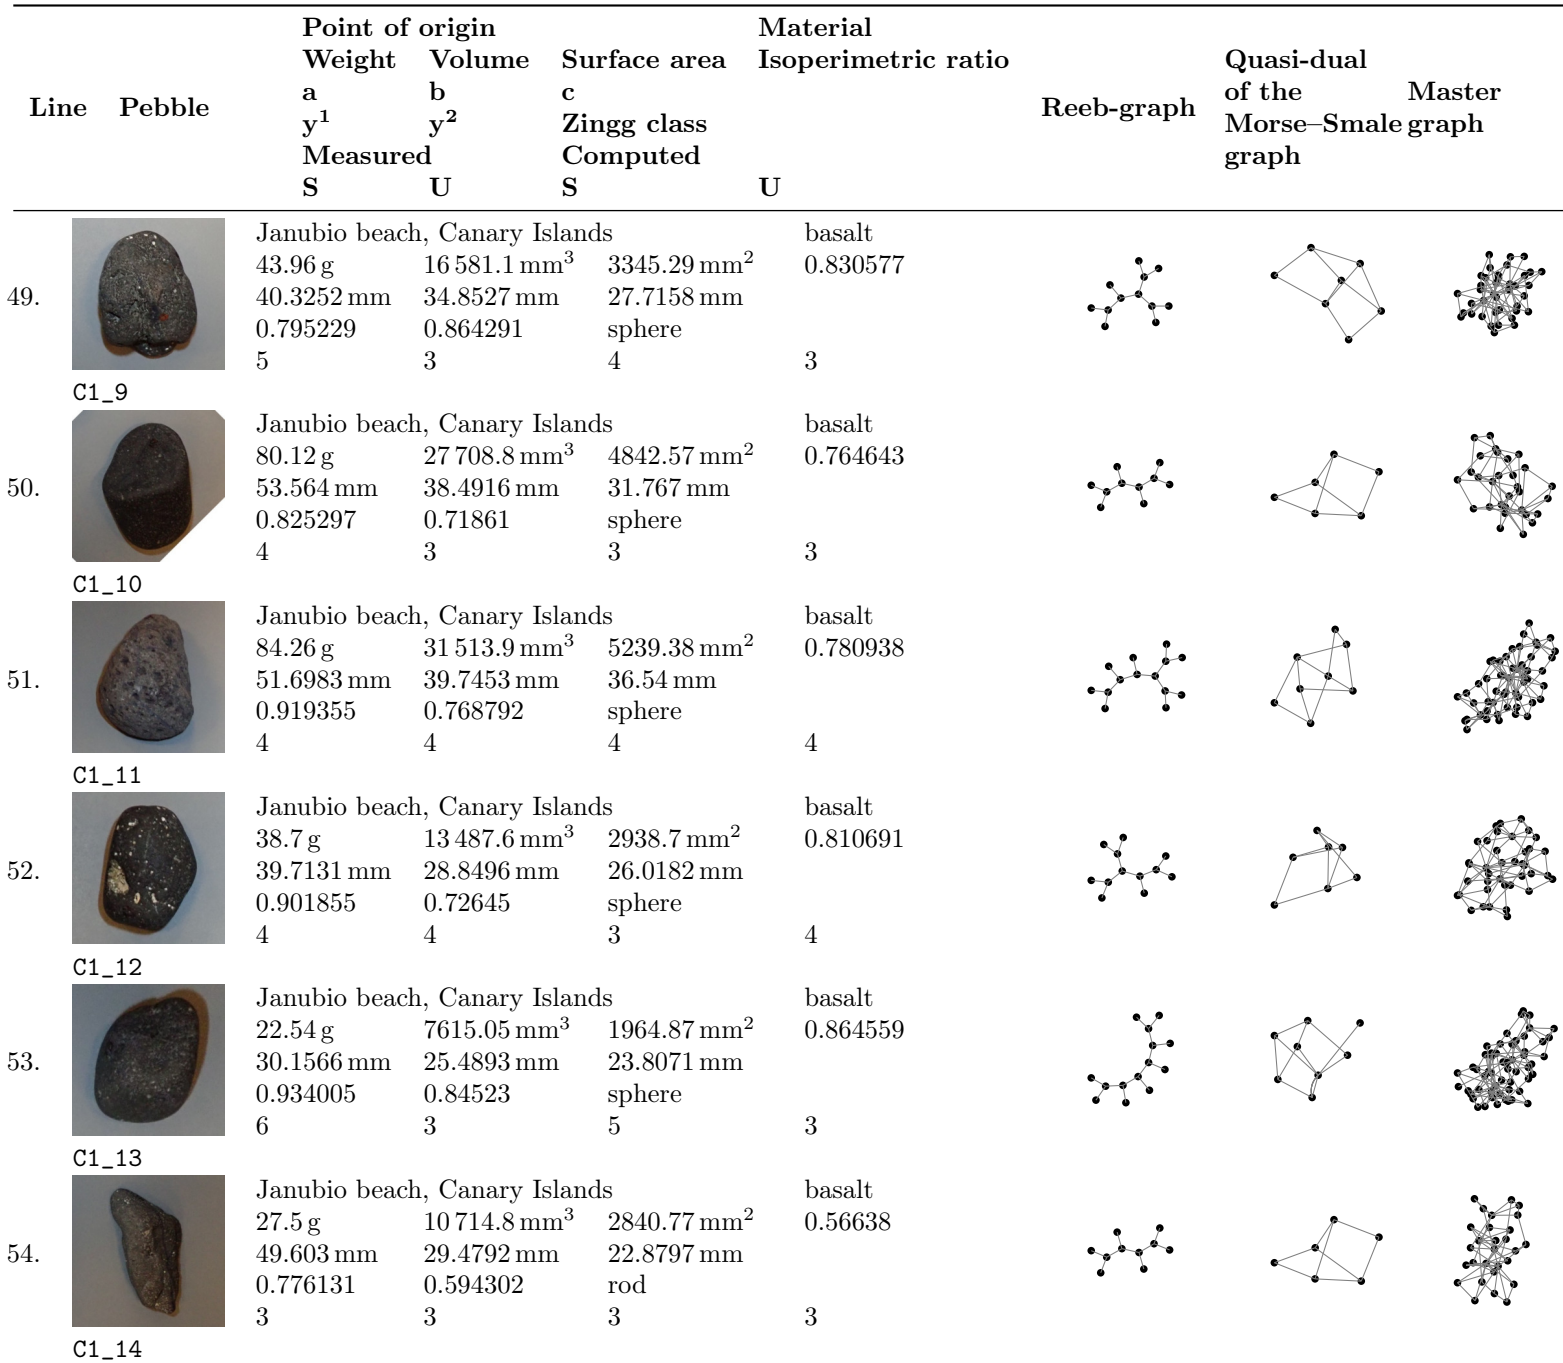  |
|      | C1_12                                                                               | 38.7 g                               | 13 487.6 mm <sup>3</sup> |                                                      |                                      |                                                                                       |                                                                                       |                                                                                       |
|      |                                                                                     | 39.7131 mm                           | 28.8496 mm               |                                                      |                                      |                                                                                       |                                                                                       |                                                                                       |
|      |                                                                                     | 0.901855                             | 0.72645                  |                                                      |                                      |                                                                                       |                                                                                       |                                                                                       |
|      |                                                                                     | 4                                    | 4                        |                                                      |                                      |                                                                                       |                                                                                       |                                                                                       |
| 53.  | 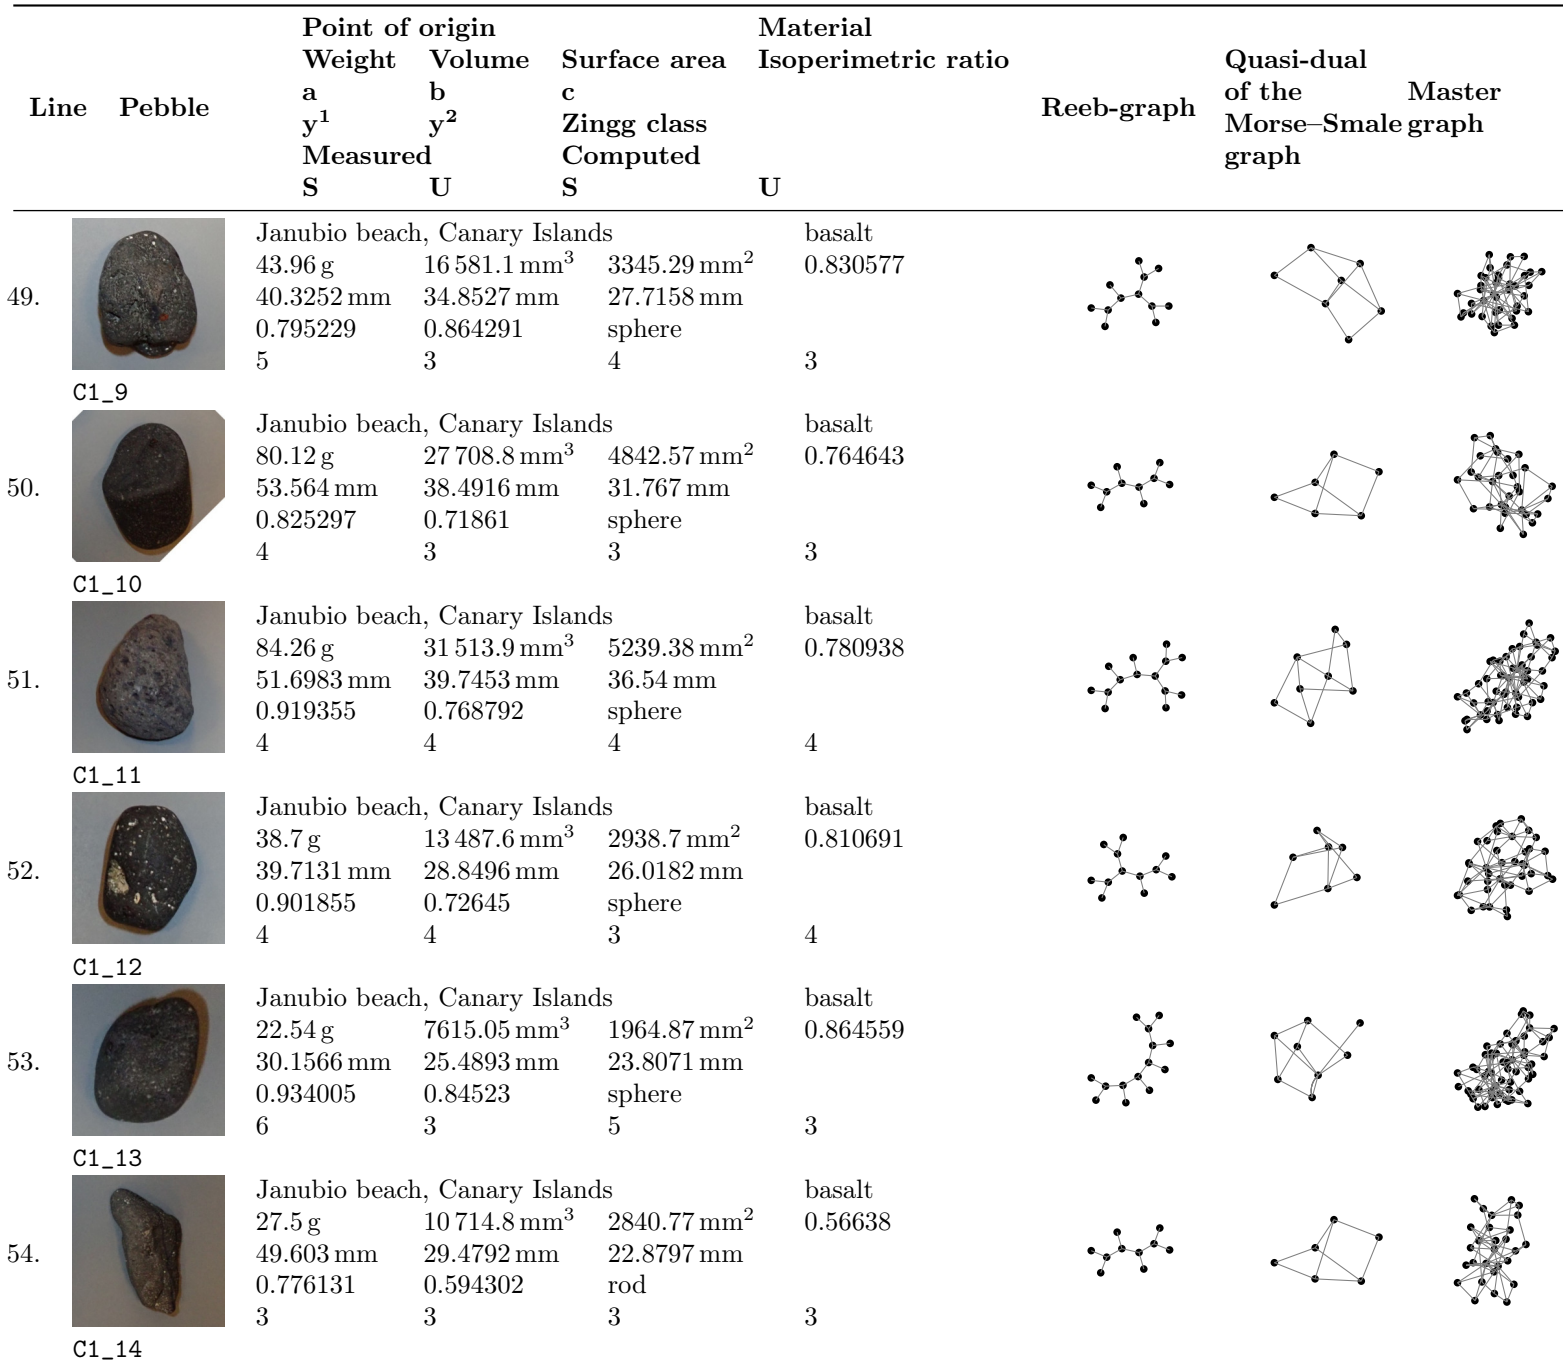 | Janubio beach, Canary Islands        |                          | 1964.87 mm <sup>2</sup><br>23.8071 mm<br>sphere<br>5 | basalt<br>0.864559<br><br>3          | 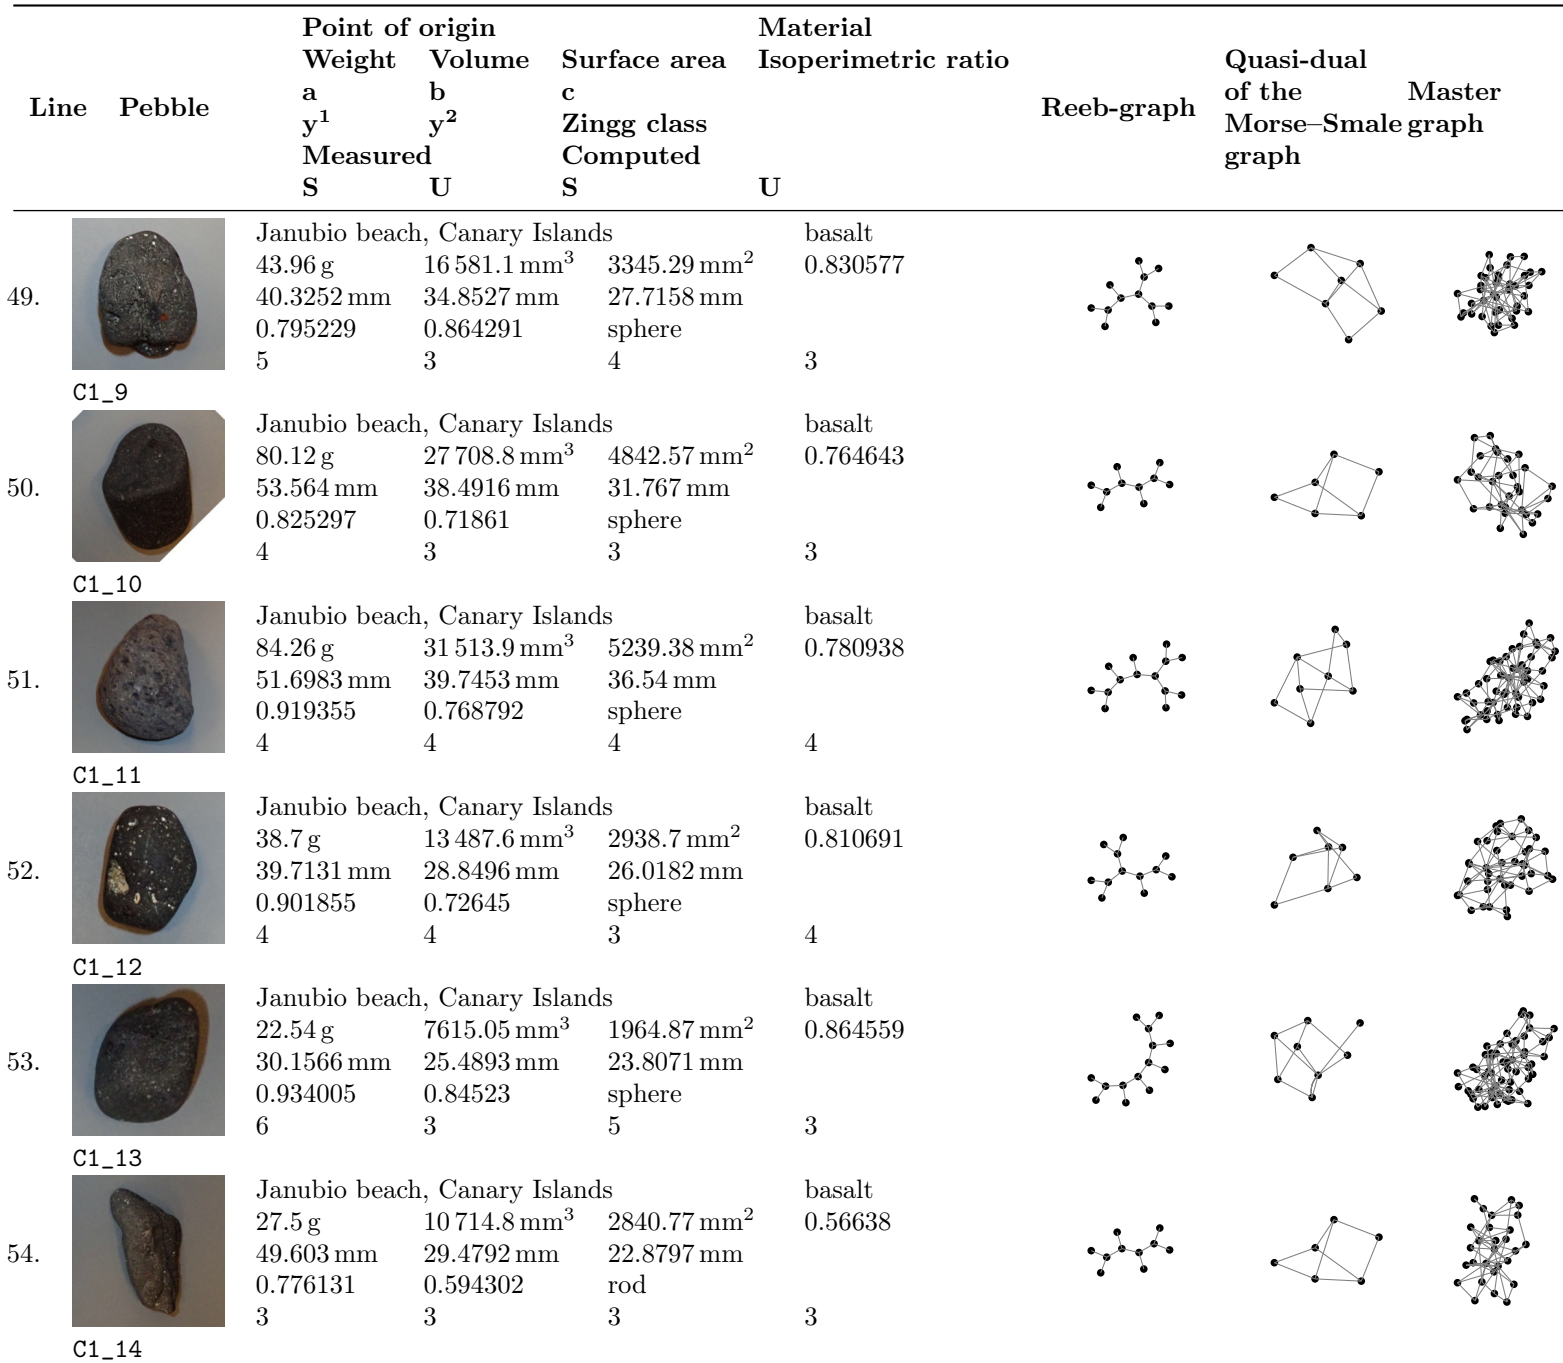 | 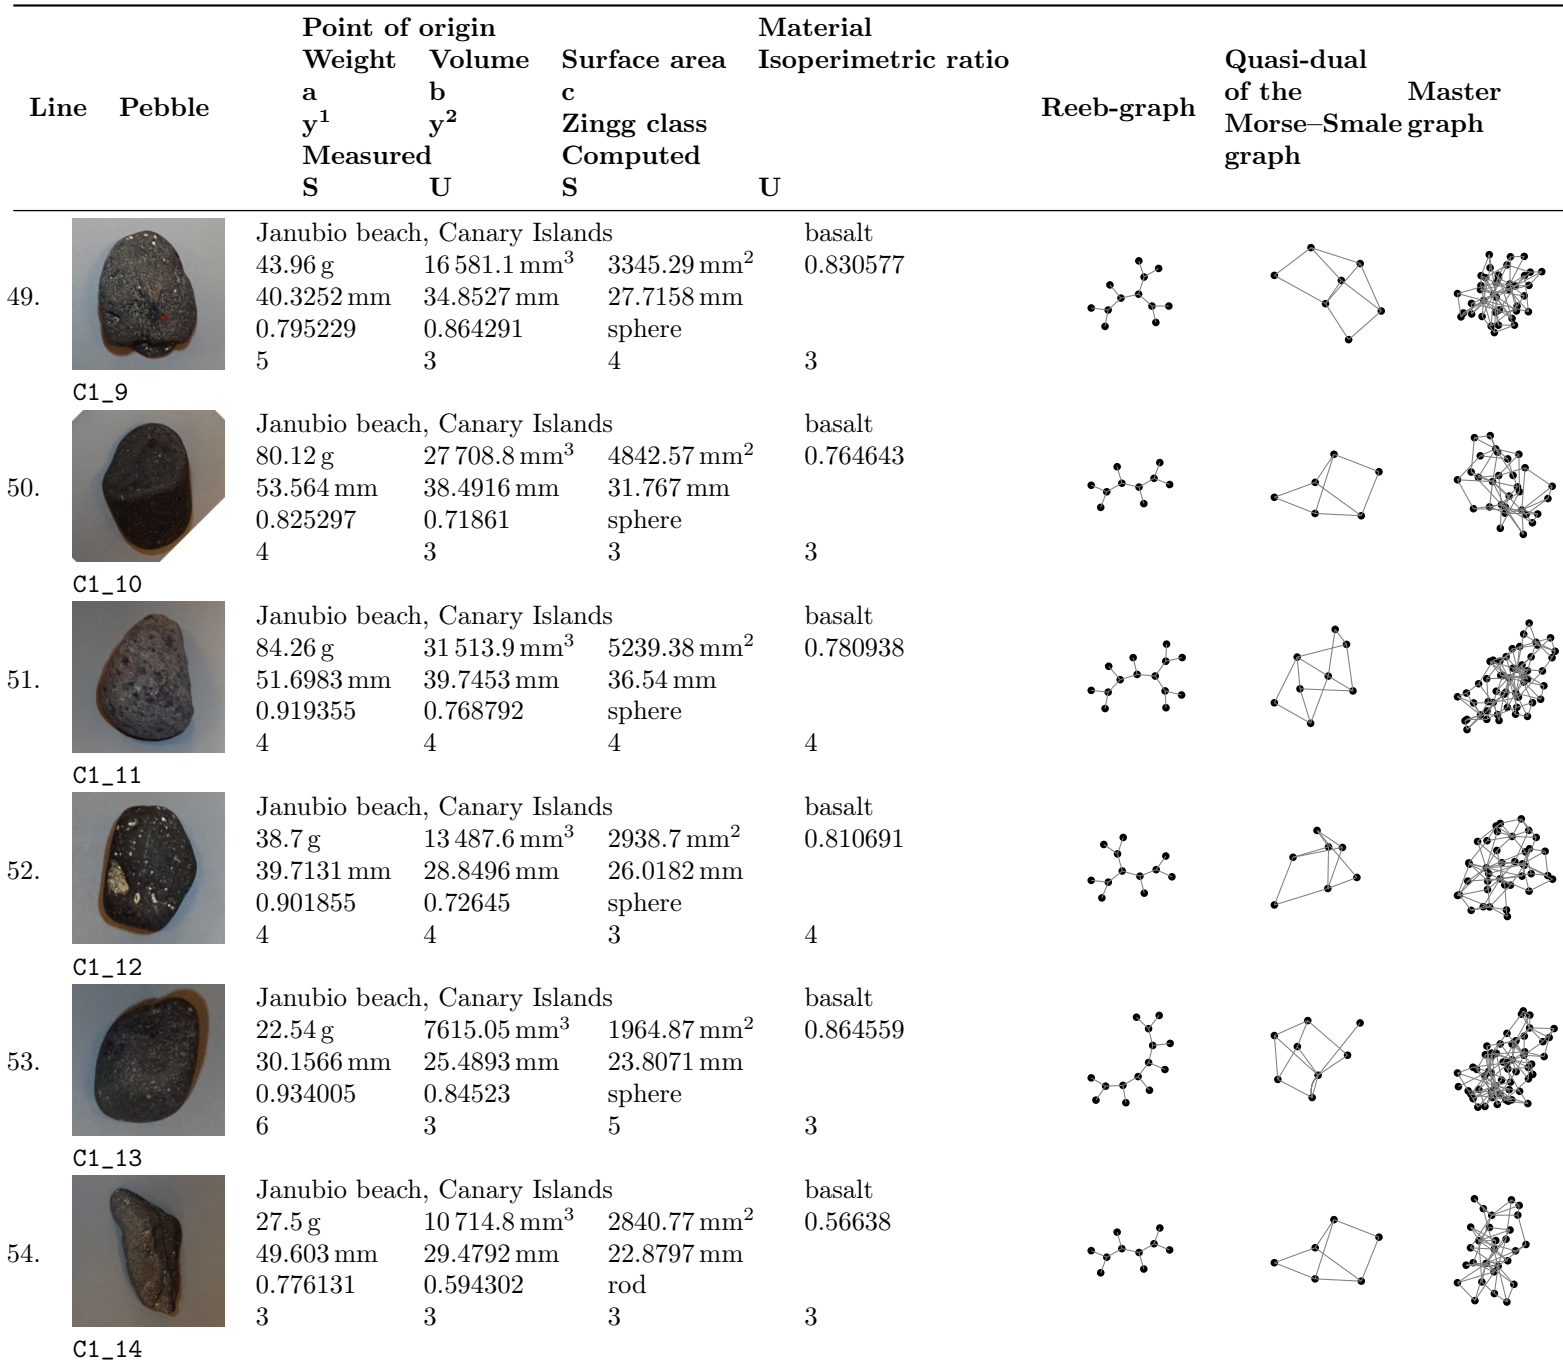 | 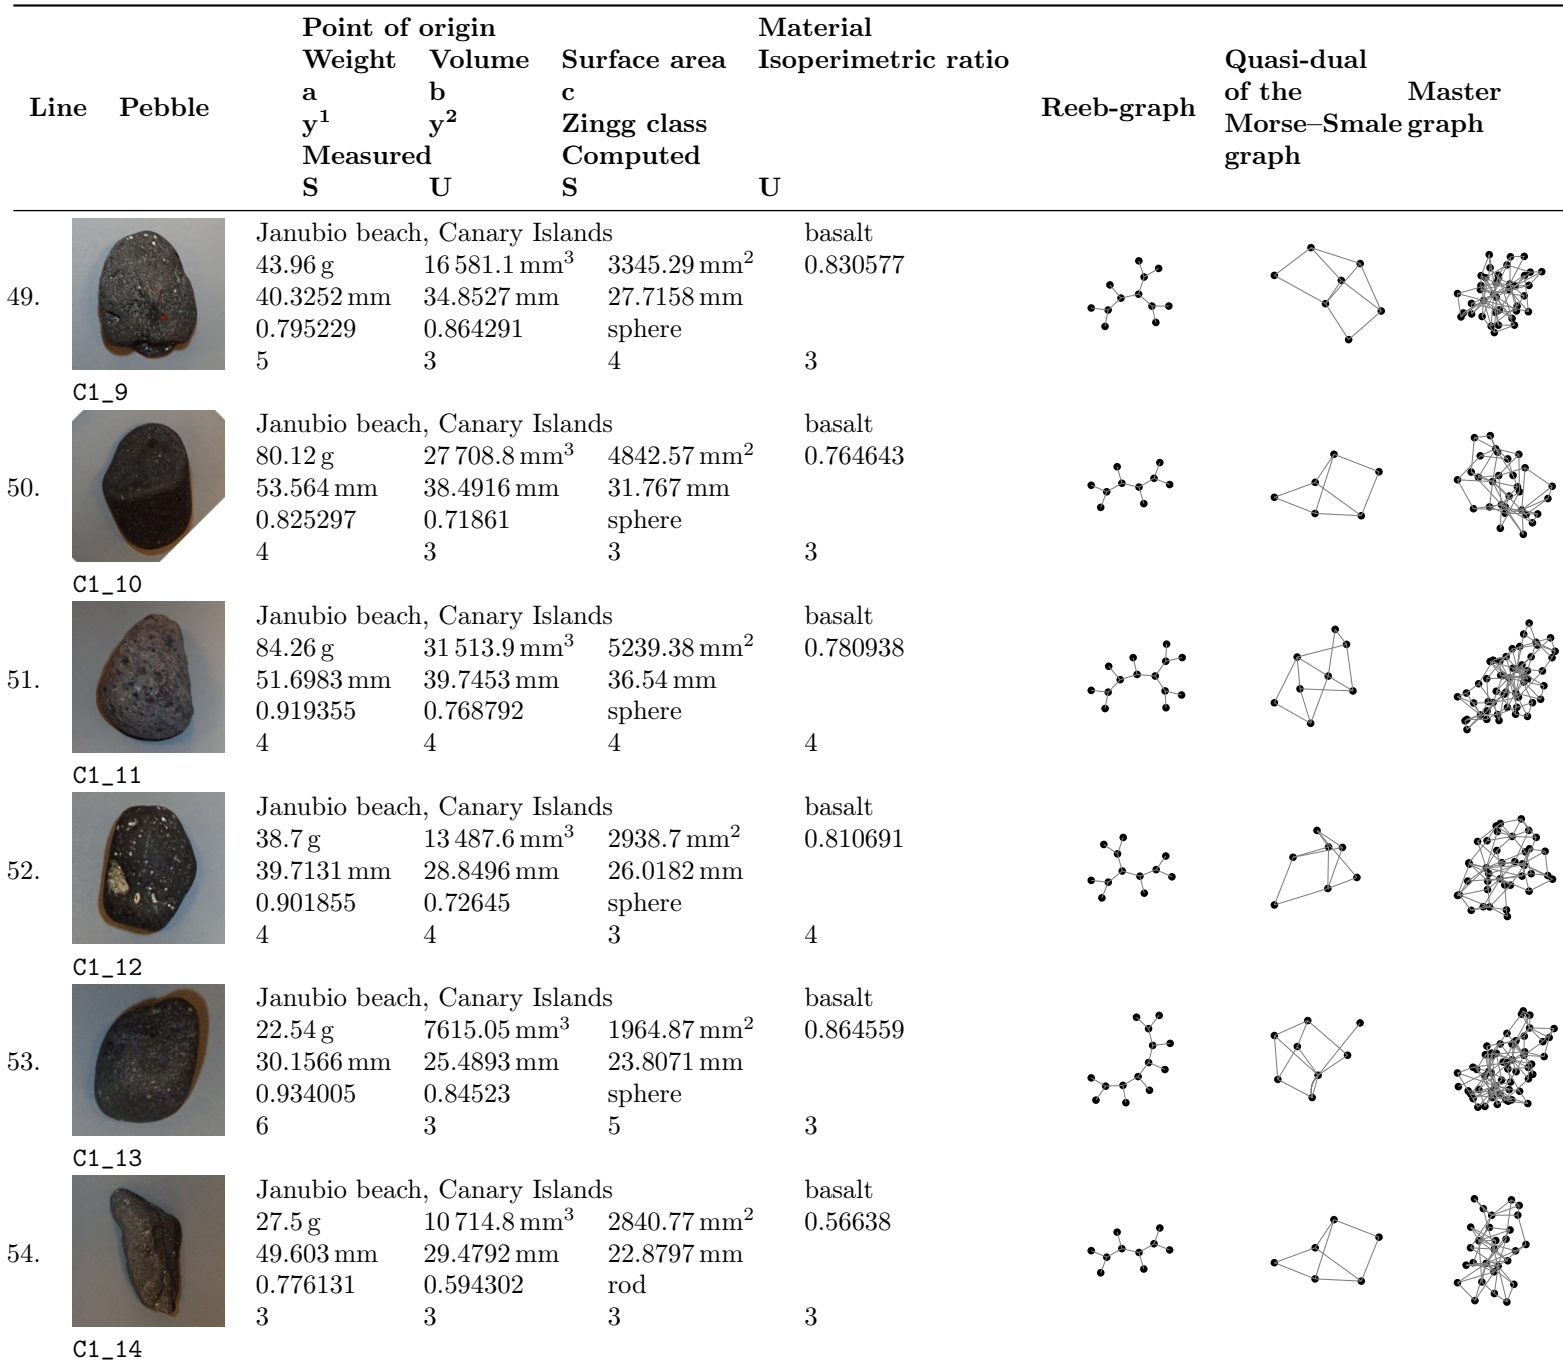 |
|      | C1_13                                                                               | 22.54 g                              | 7615.05 mm <sup>3</sup>  |                                                      |                                      |                                                                                       |                                                                                       |                                                                                       |
|      |                                                                                     | 30.1566 mm                           | 25.4893 mm               |                                                      |                                      |                                                                                       |                                                                                       |                                                                                       |
|      |                                                                                     | 0.934005                             | 0.84523                  |                                                      |                                      |                                                                                       |                                                                                       |                                                                                       |
|      |                                                                                     | 6                                    | 3                        |                                                      |                                      |                                                                                       |                                                                                       |                                                                                       |
| 54.  | 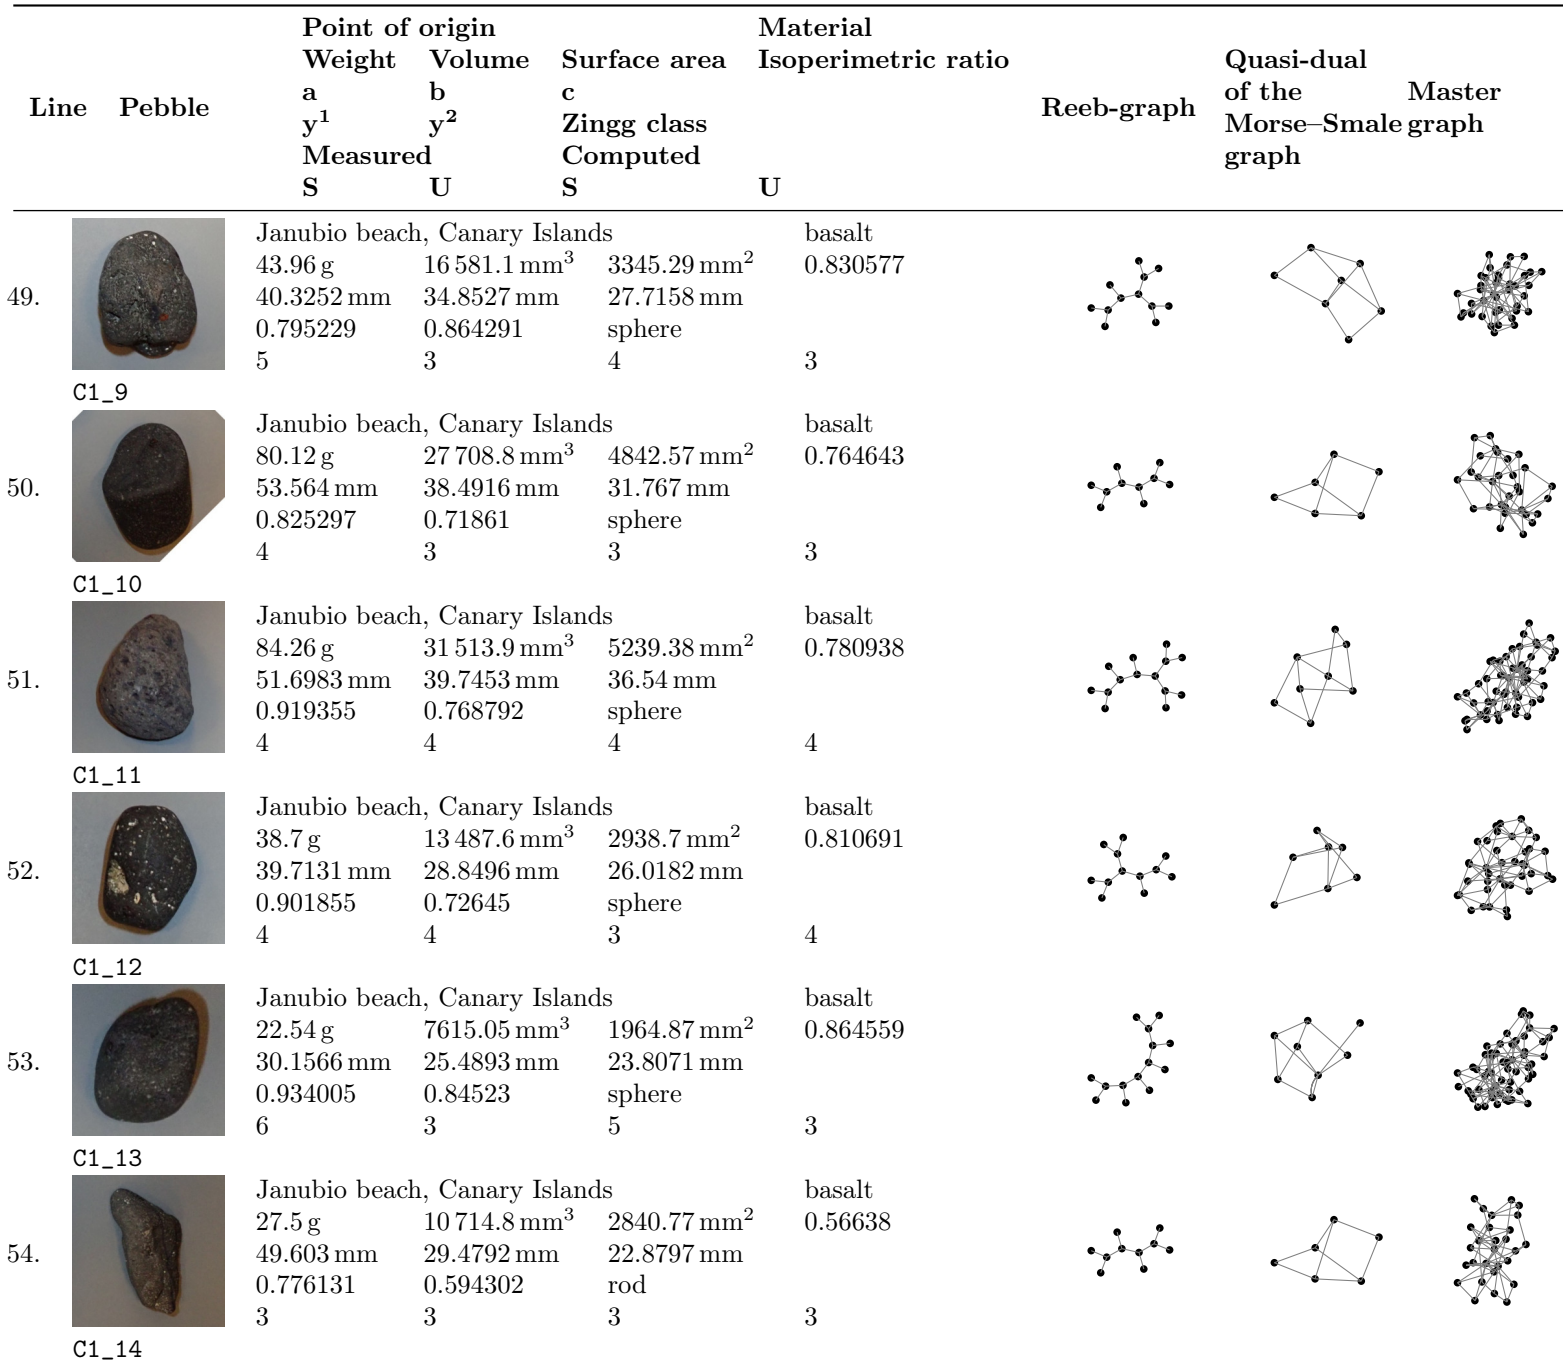 | Janubio beach, Canary Islands        |                          | 2840.77 mm <sup>2</sup><br>22.8797 mm<br>rod<br>3    | basalt<br>0.56638<br><br>3           | 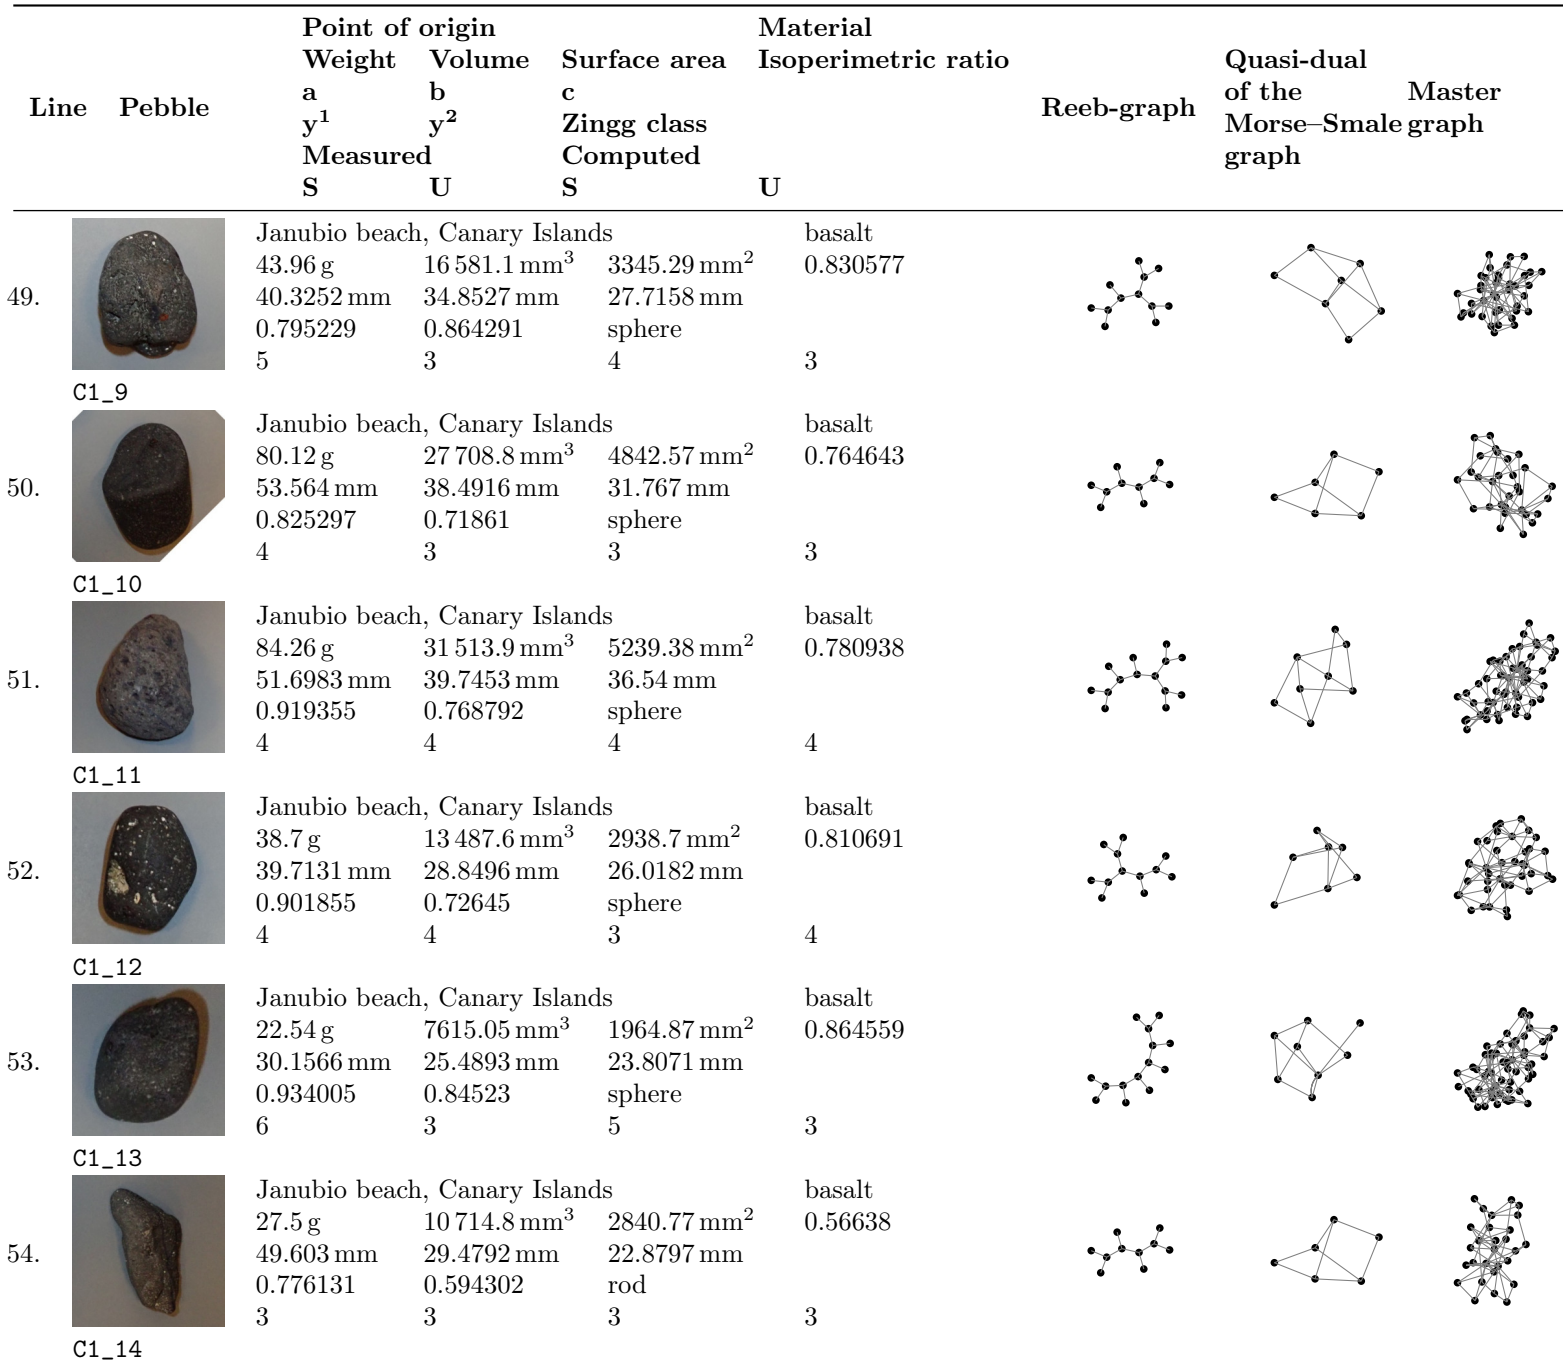 | 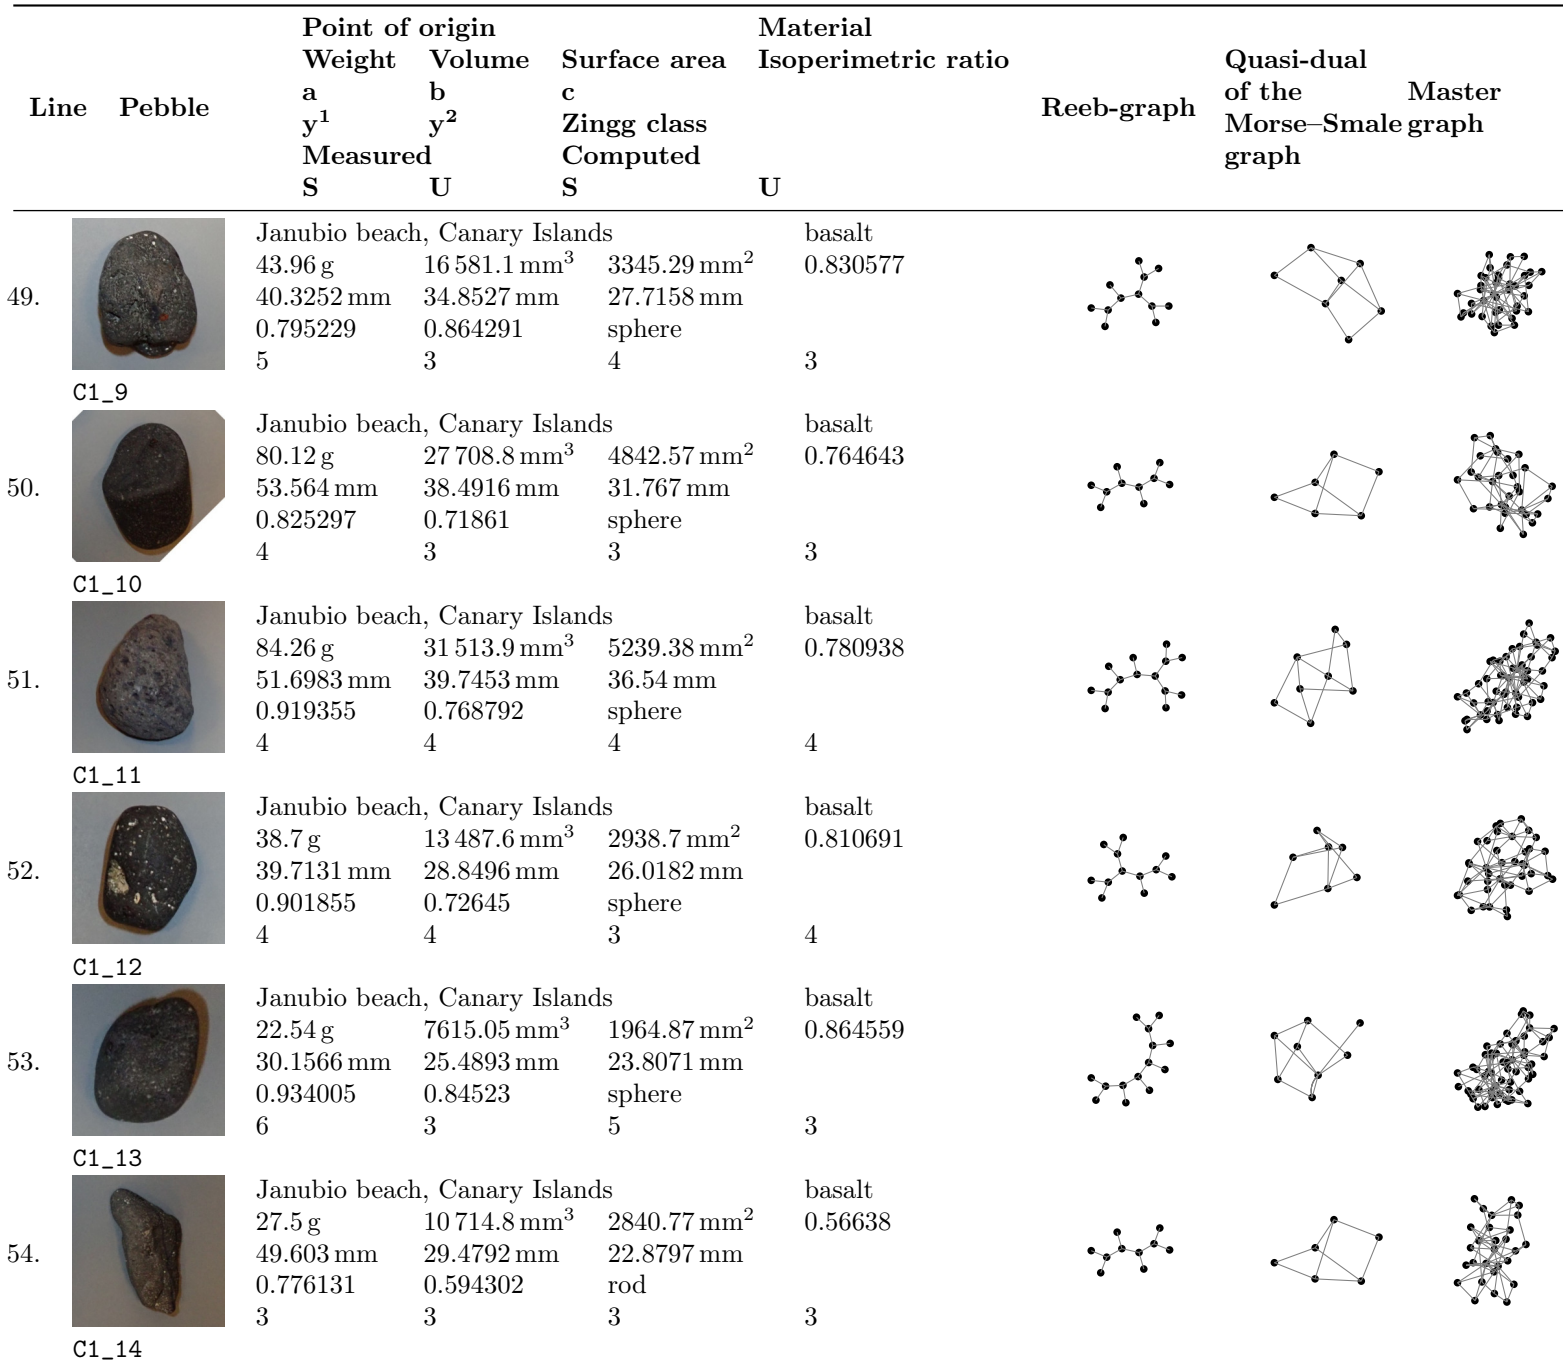 | 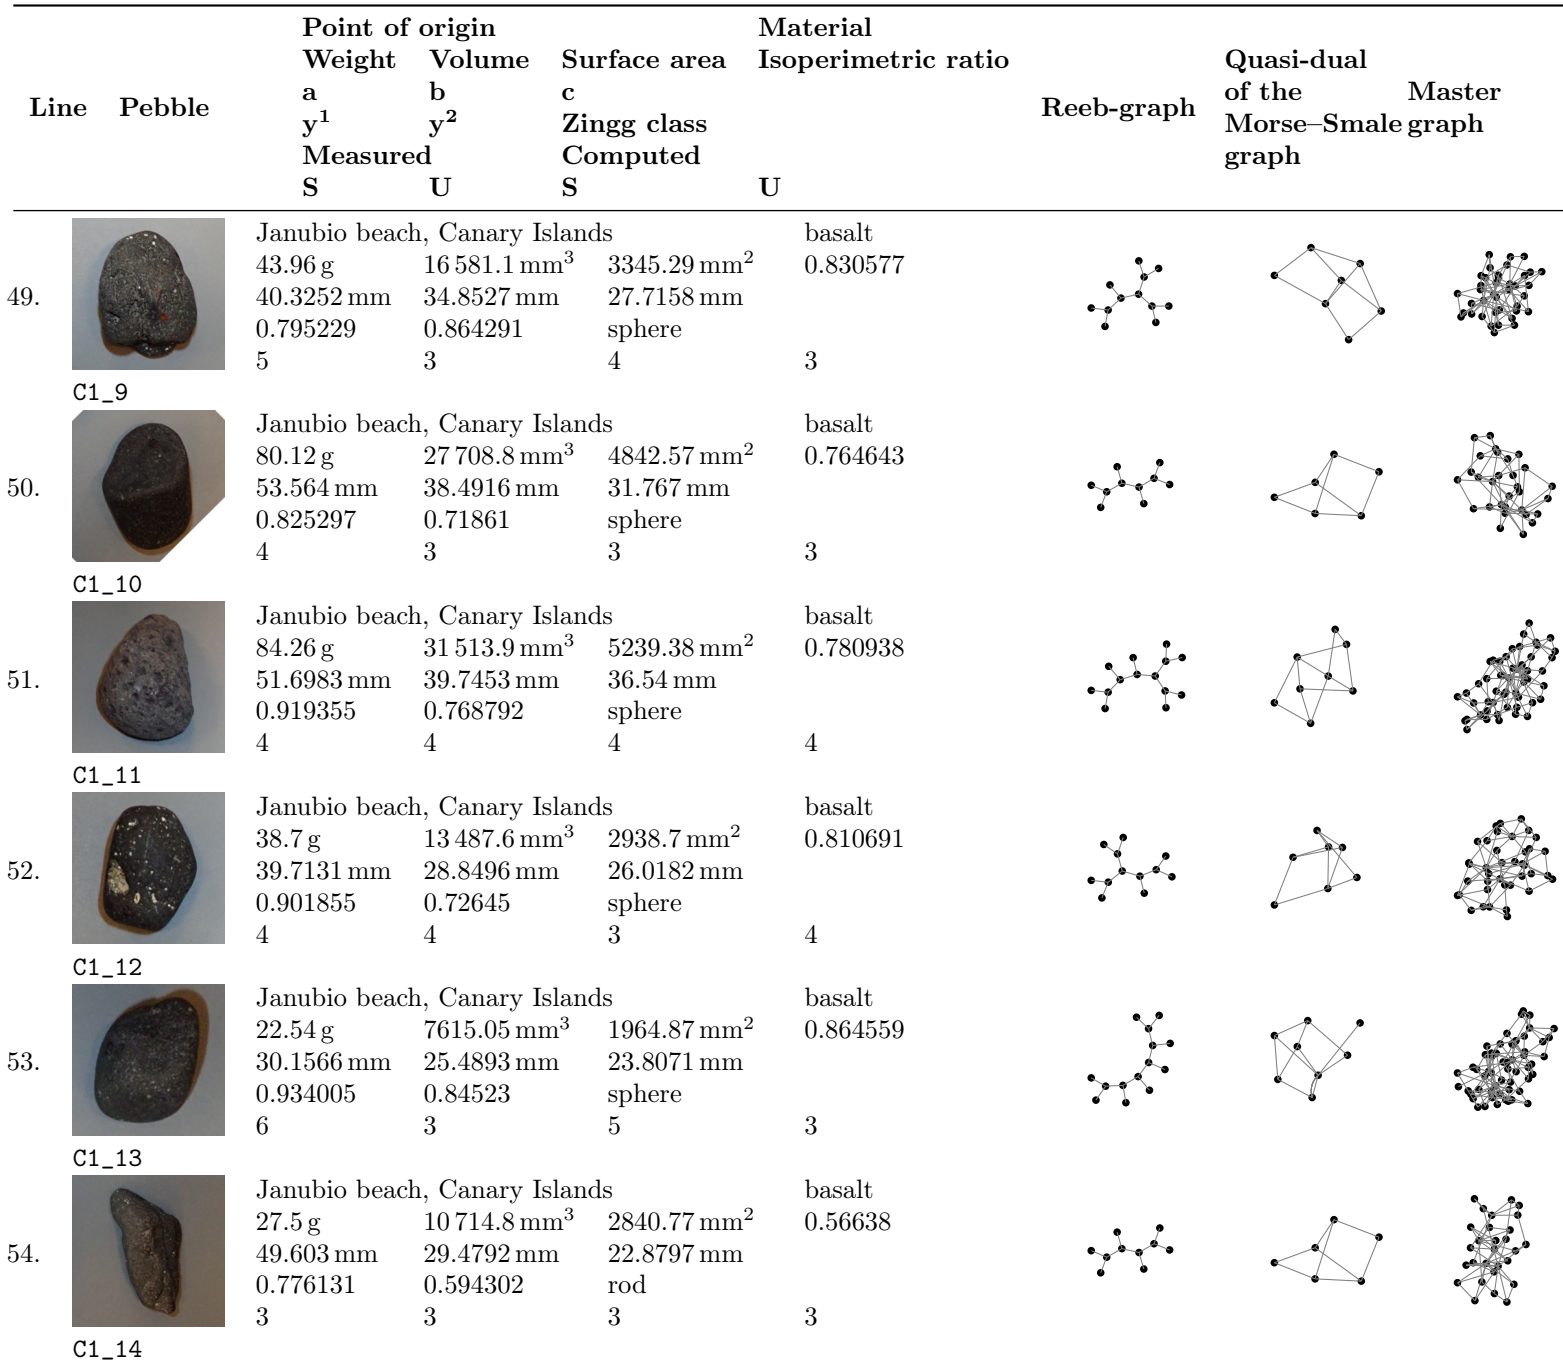 |
|      | C1_14                                                                               | 27.5 g                               | 10 714.8 mm <sup>3</sup> |                                                      |                                      |                                                                                       |                                                                                       |                                                                                       |
|      |                                                                                     | 49.603 mm                            | 29.4792 mm               |                                                      |                                      |                                                                                       |                                                                                       |                                                                                       |
|      |                                                                                     | 0.776131                             | 0.594302                 |                                                      |                                      |                                                                                       |                                                                                       |                                                                                       |
|      |                                                                                     | 3                                    | 3                        |                                                      |                                      |                                                                                       |                                                                                       |                                                                                       |

| Line  | Pebble                                                                              | Point of origin                      |                          |                                   | Material | Isoperimetric ratio                                                                   | Reeb-graph                                                                            | Quasi-dual<br>of the<br>Morse–Smale graph                                             | Master<br>graph |
|-------|-------------------------------------------------------------------------------------|--------------------------------------|--------------------------|-----------------------------------|----------|---------------------------------------------------------------------------------------|---------------------------------------------------------------------------------------|---------------------------------------------------------------------------------------|-----------------|
|       |                                                                                     | Weight                               | Volume                   | Surface area                      |          |                                                                                       |                                                                                       |                                                                                       |                 |
|       |                                                                                     | a<br>y <sup>1</sup><br>Measured<br>S | b<br>y <sup>2</sup><br>U | c<br>Zingg class<br>Computed<br>S |          |                                                                                       |                                                                                       |                                                                                       |                 |
|       |                                                                                     |                                      |                          | U                                 |          |                                                                                       |                                                                                       |                                                                                       |                 |
| 55.   | 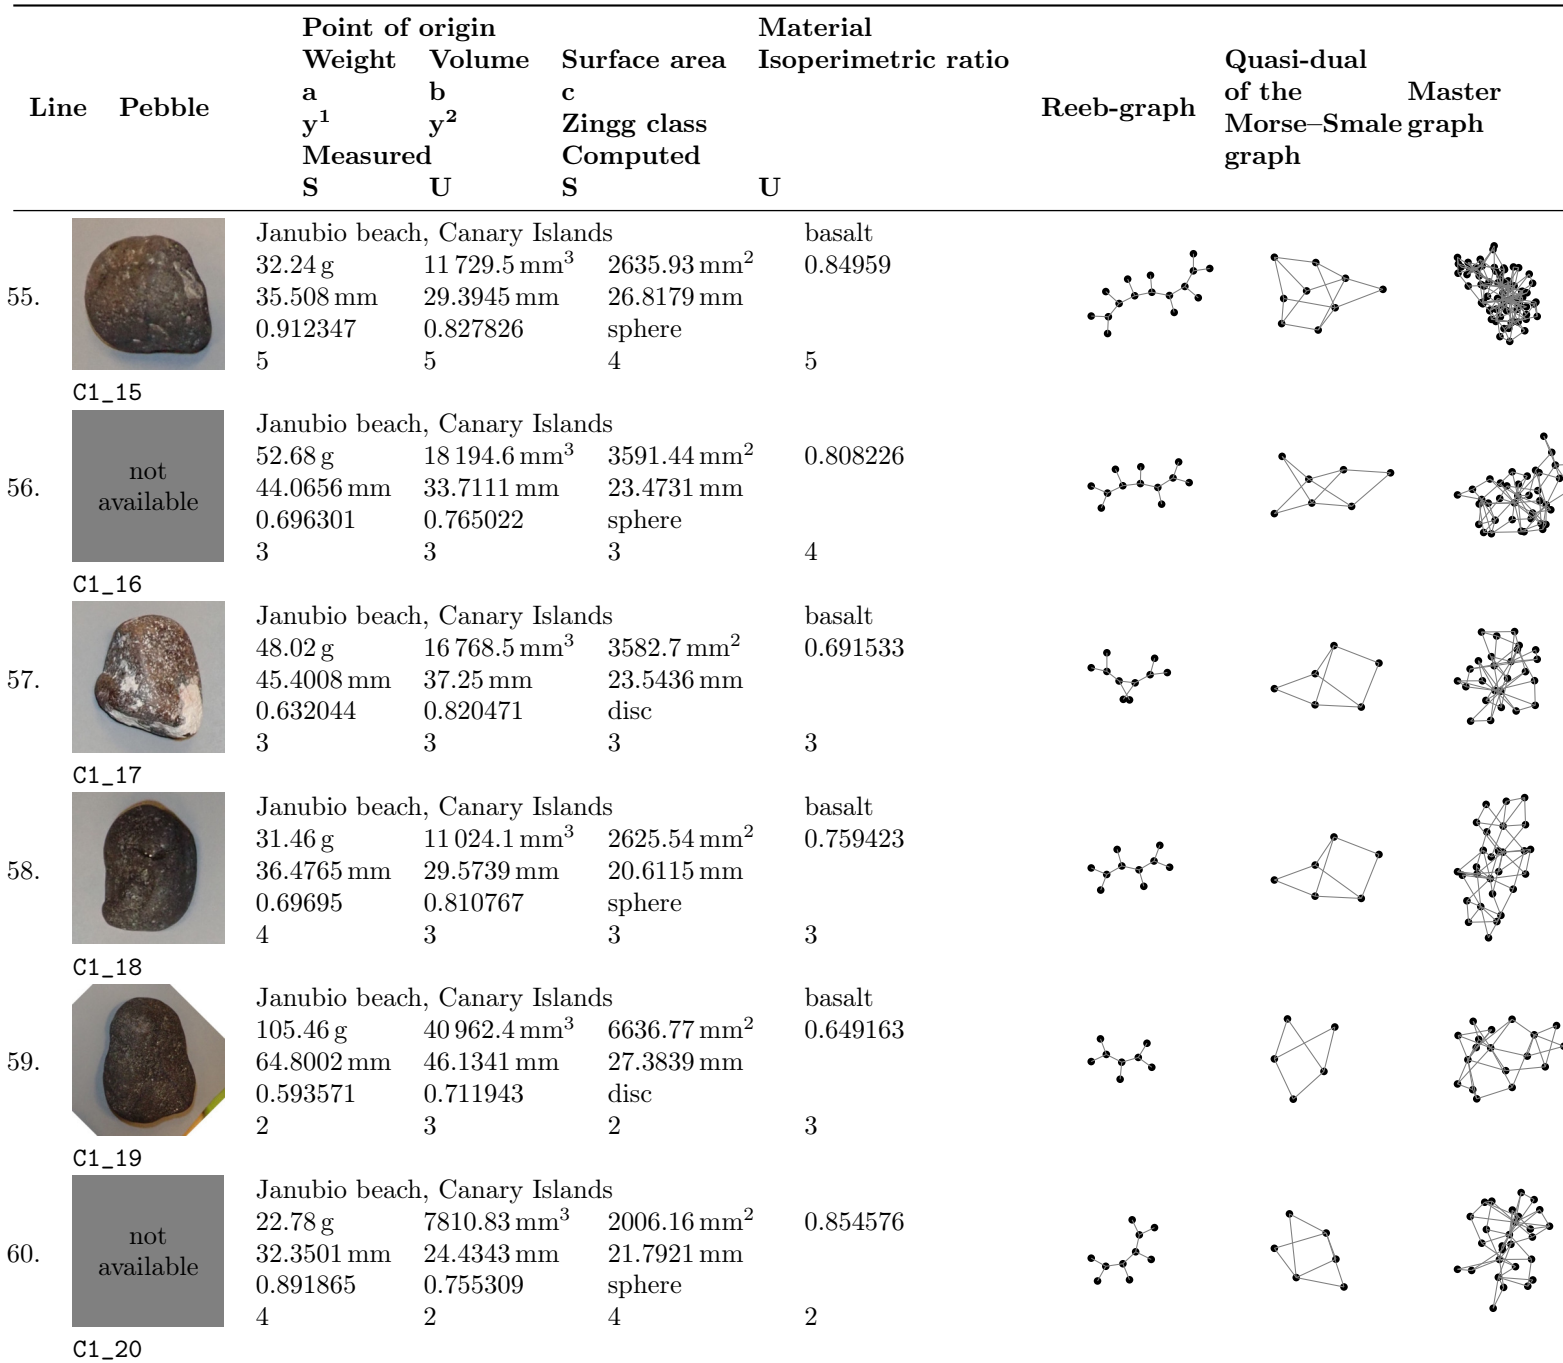   | Janubio beach, Canary Islands        |                          |                                   | basalt   | 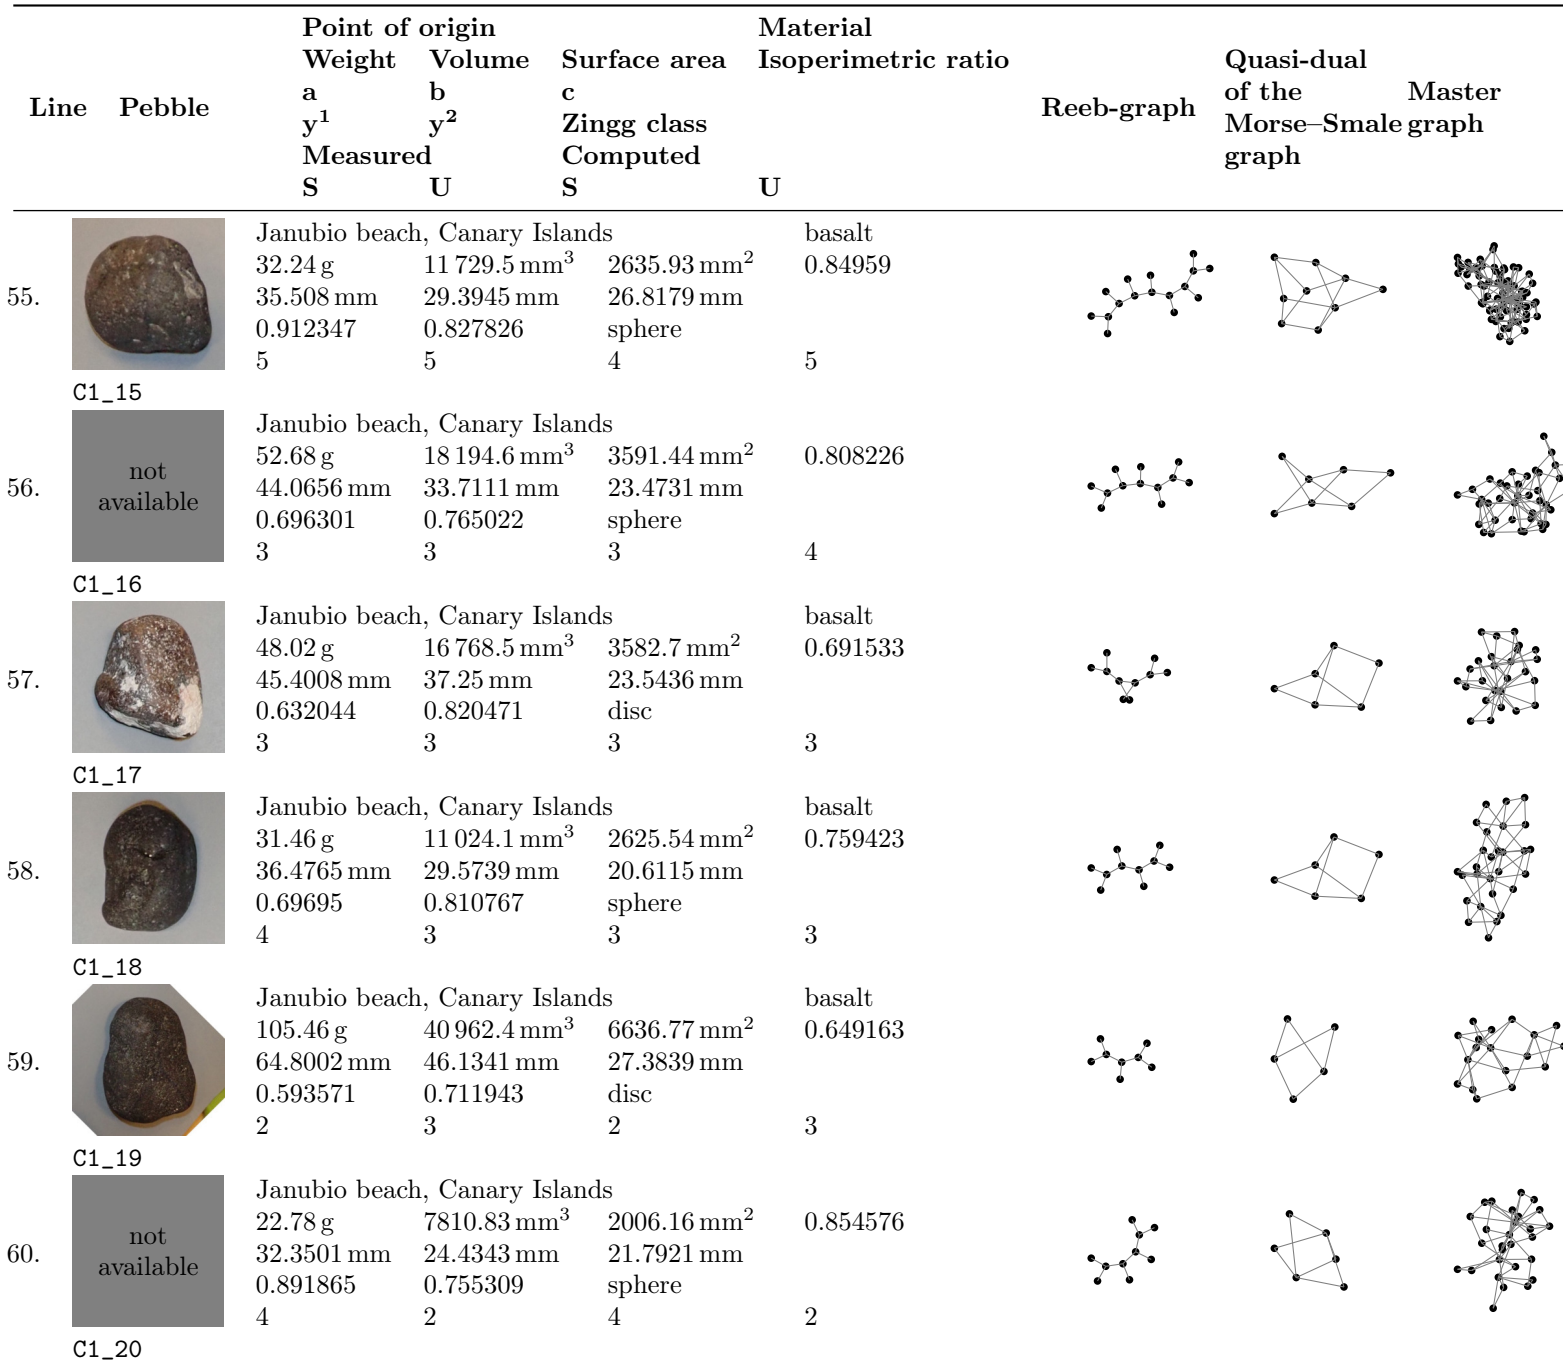   | 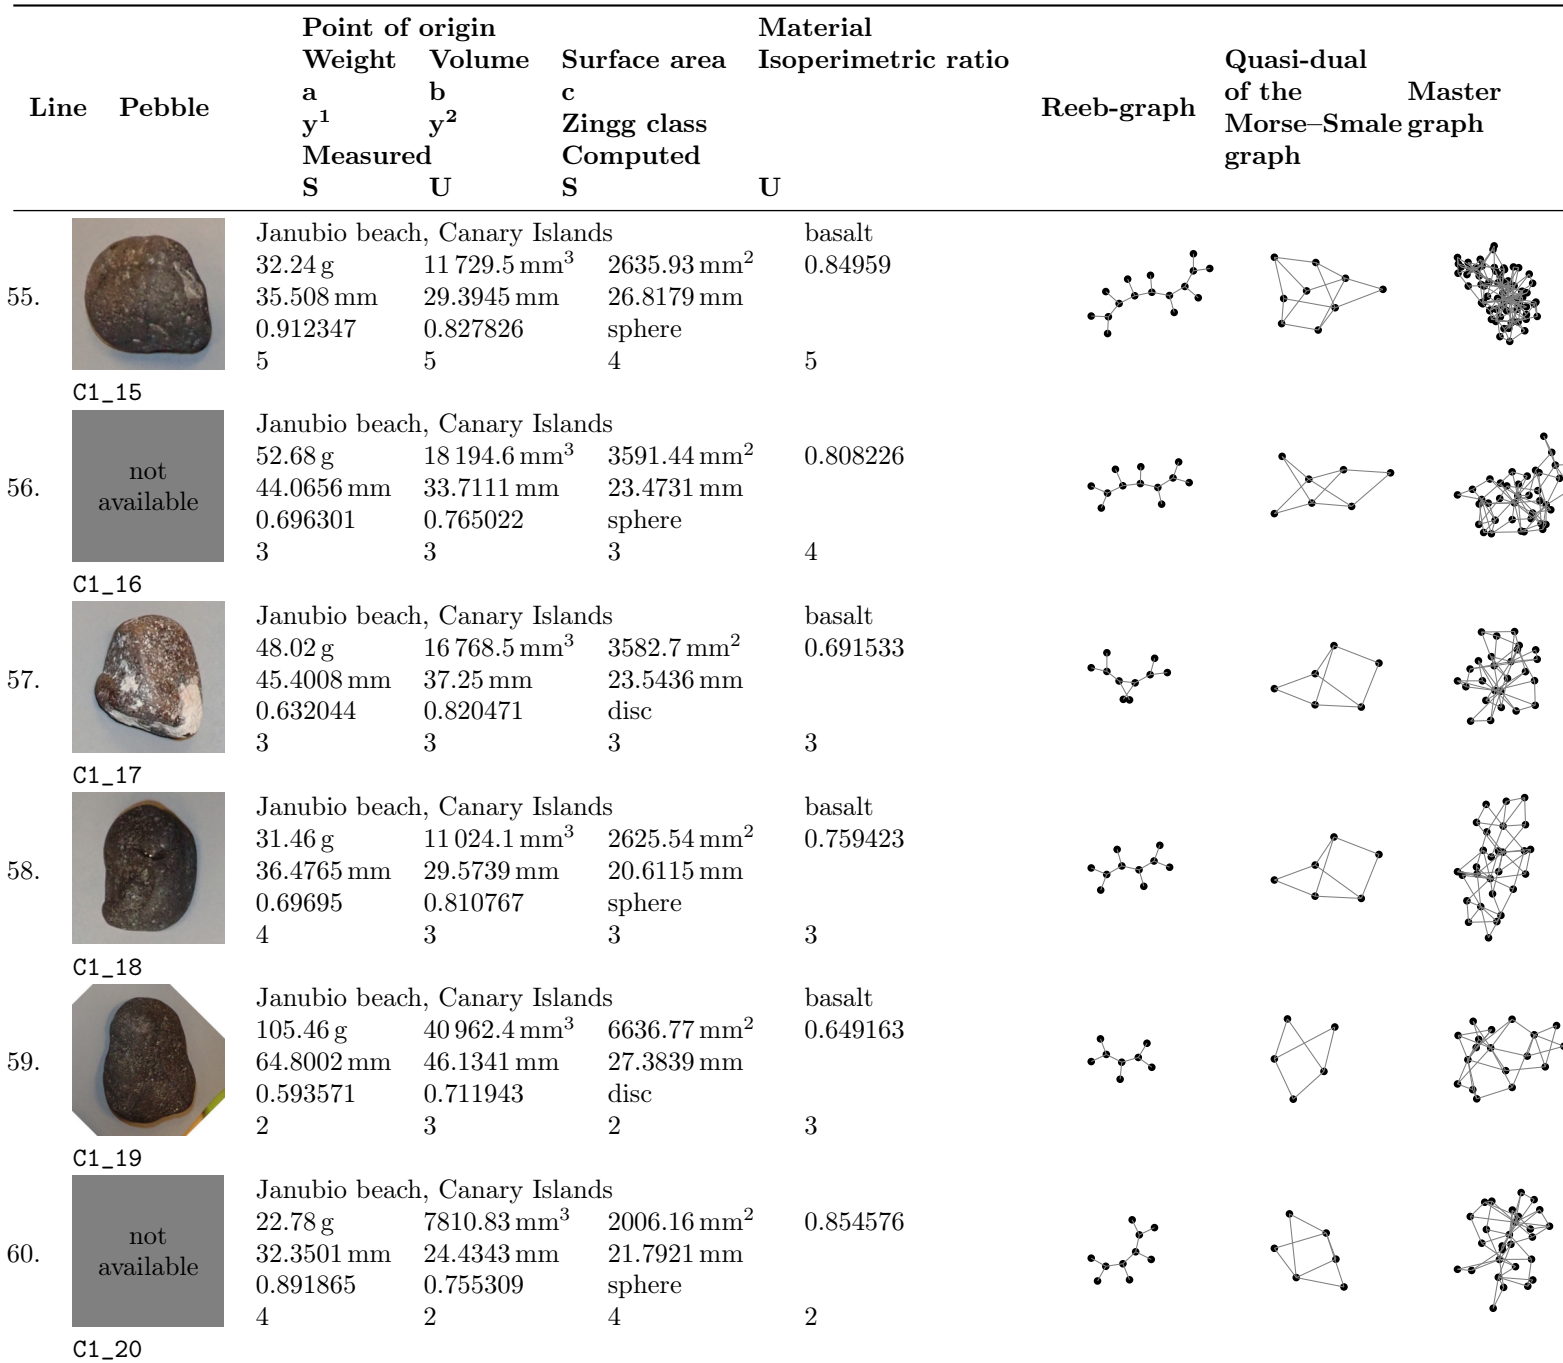   | 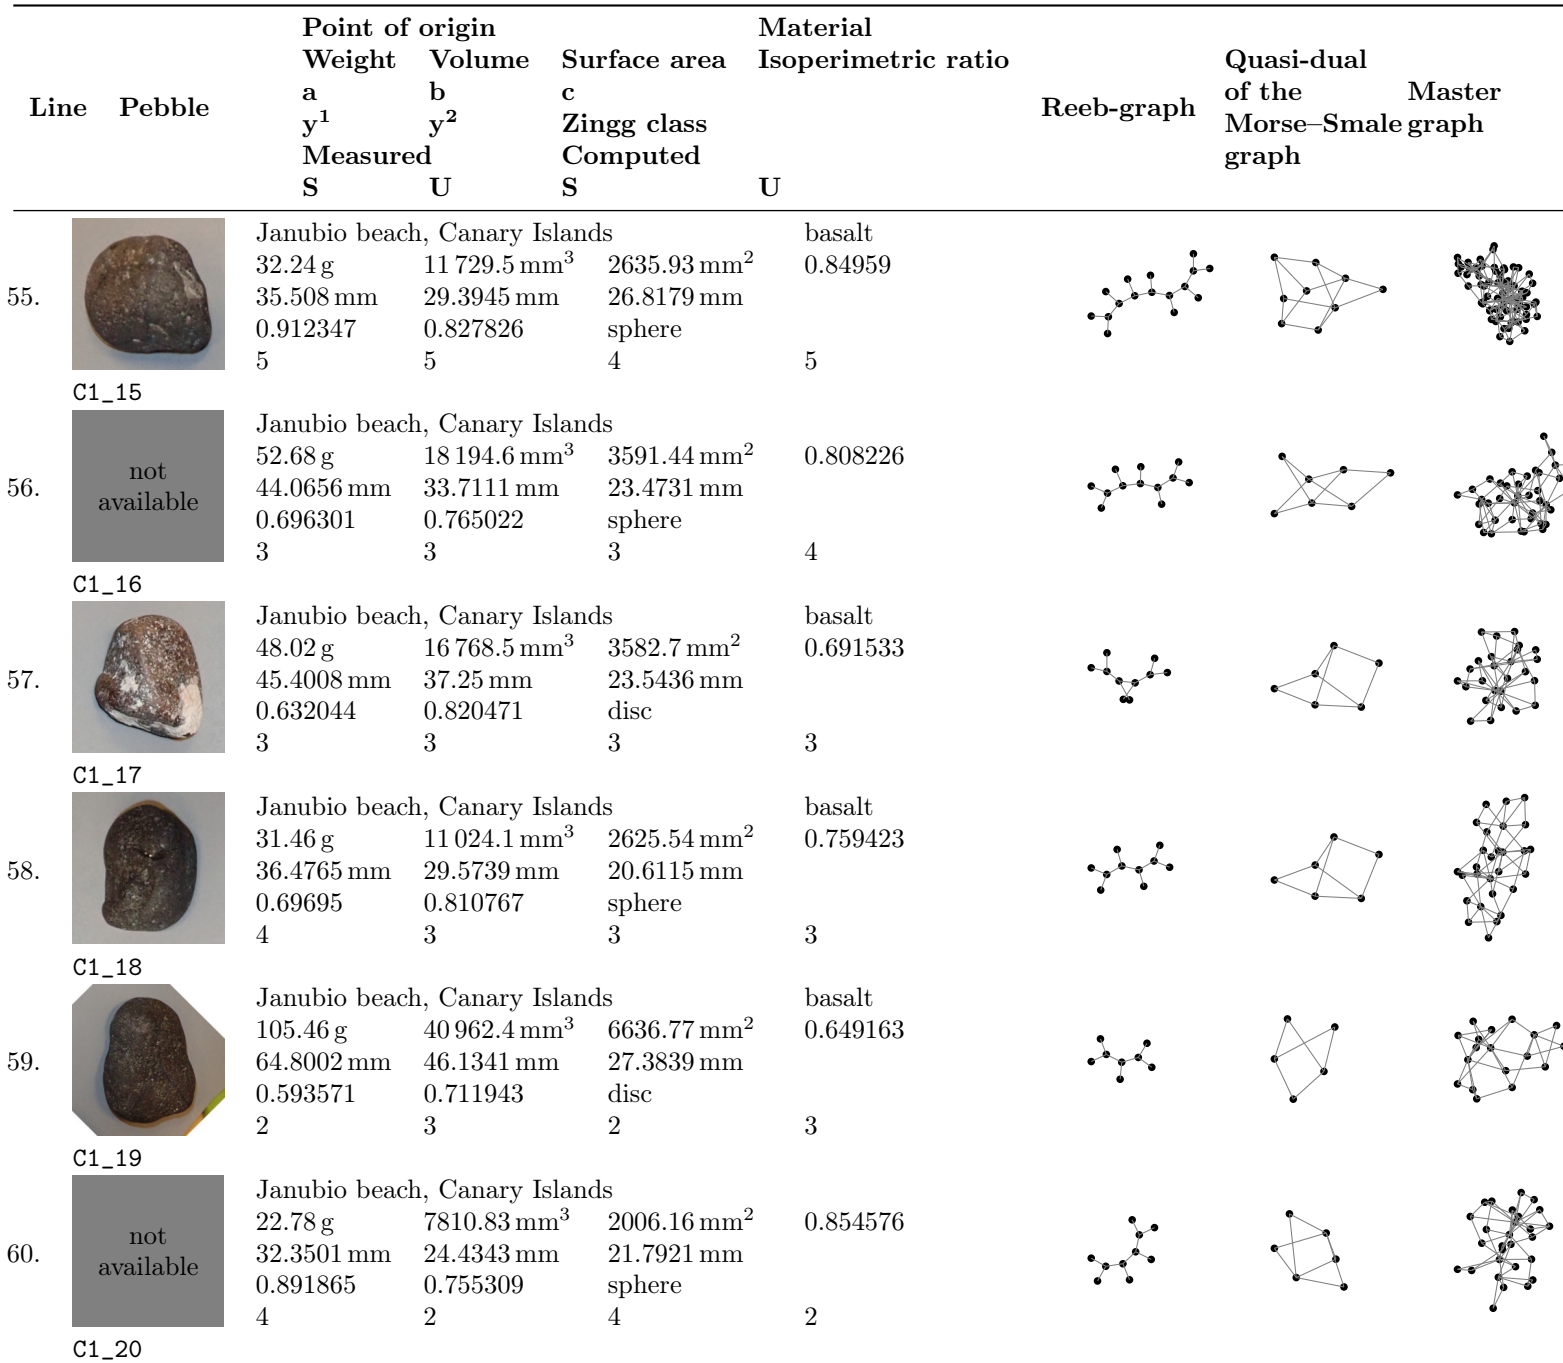   |                 |
|       | 32.24 g                                                                             | 11 729.5 mm <sup>3</sup>             | 2635.93 mm <sup>2</sup>  | 0.84959                           |          |                                                                                       |                                                                                       |                                                                                       |                 |
|       | 35.508 mm                                                                           | 29.3945 mm                           | 26.8179 mm               |                                   |          |                                                                                       |                                                                                       |                                                                                       |                 |
|       | 0.912347                                                                            | 0.827826                             | sphere                   |                                   |          |                                                                                       |                                                                                       |                                                                                       |                 |
|       | 5                                                                                   | 5                                    | 4                        | 5                                 |          |                                                                                       |                                                                                       |                                                                                       |                 |
| C1_15 |                                                                                     |                                      |                          |                                   |          |                                                                                       |                                                                                       |                                                                                       |                 |
| 56.   | 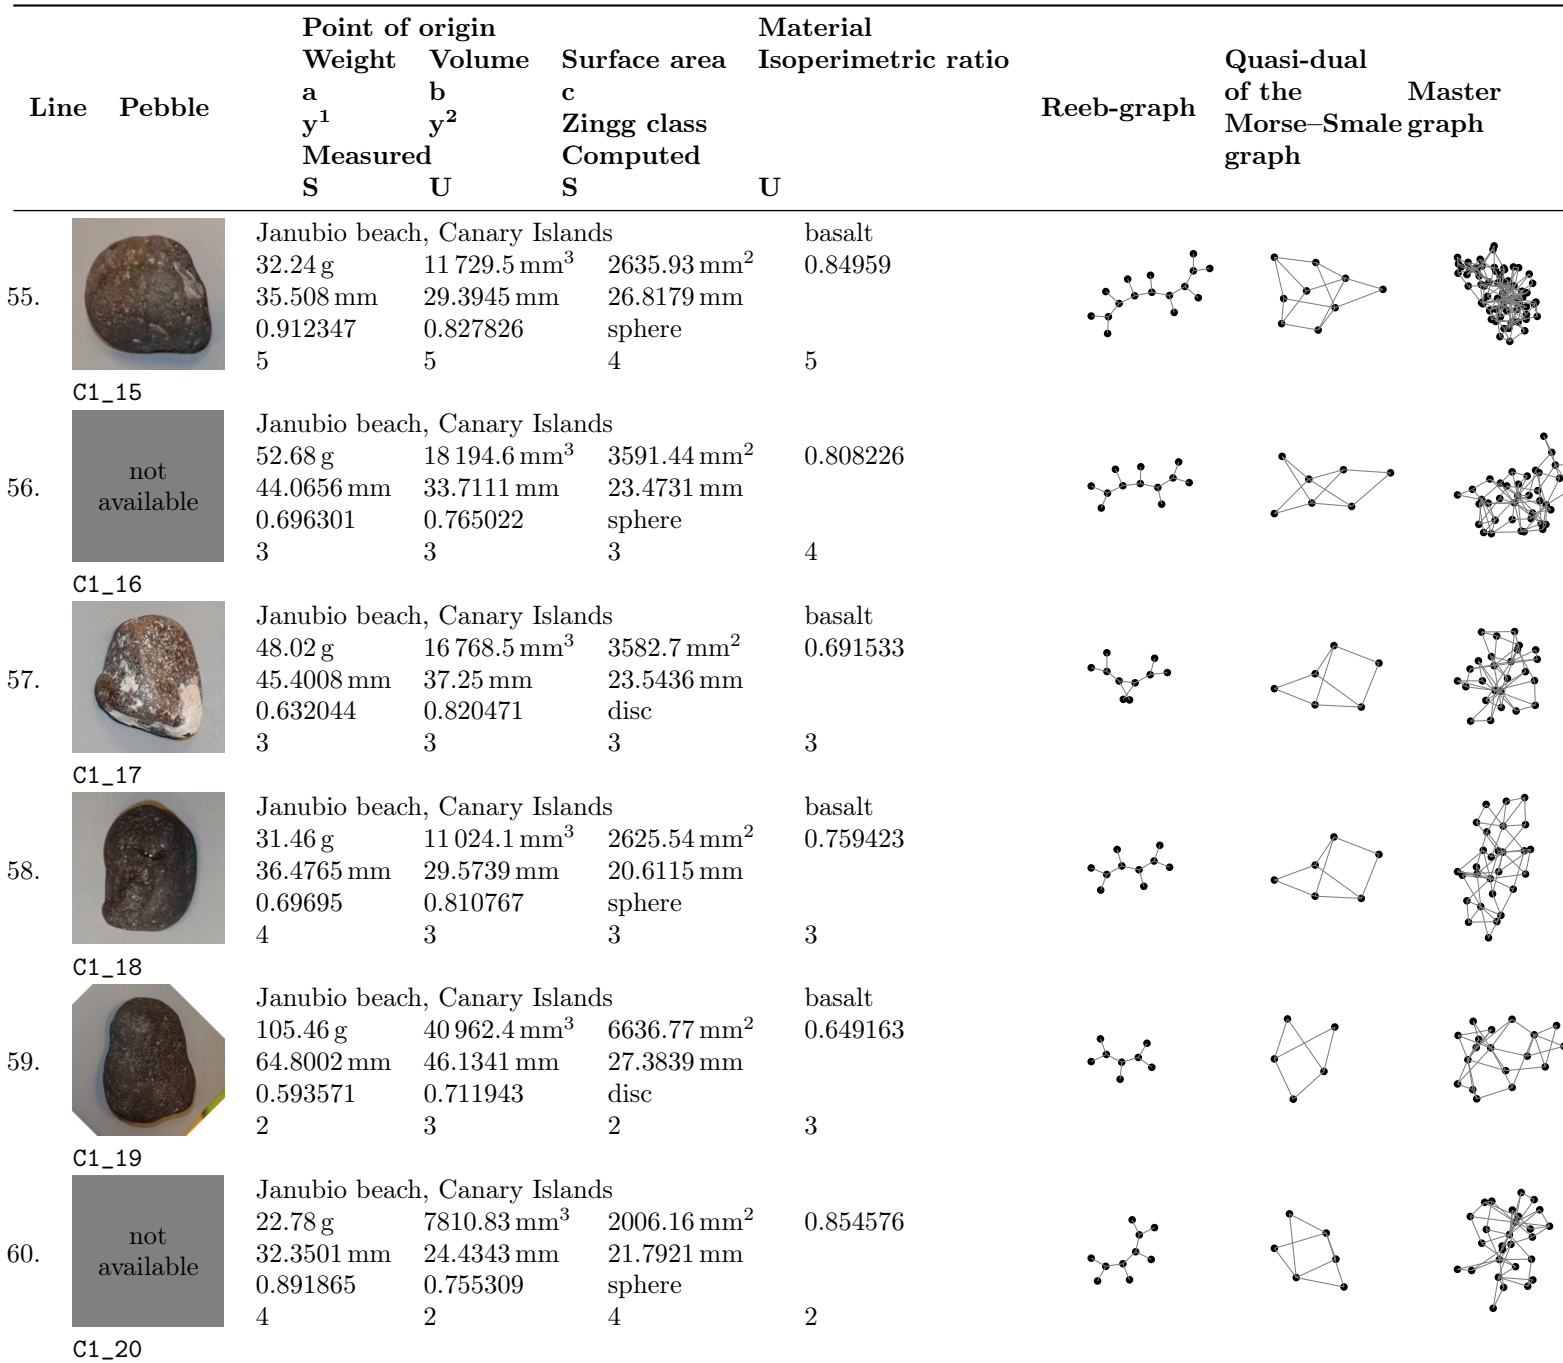   | Janubio beach, Canary Islands        |                          |                                   |          | 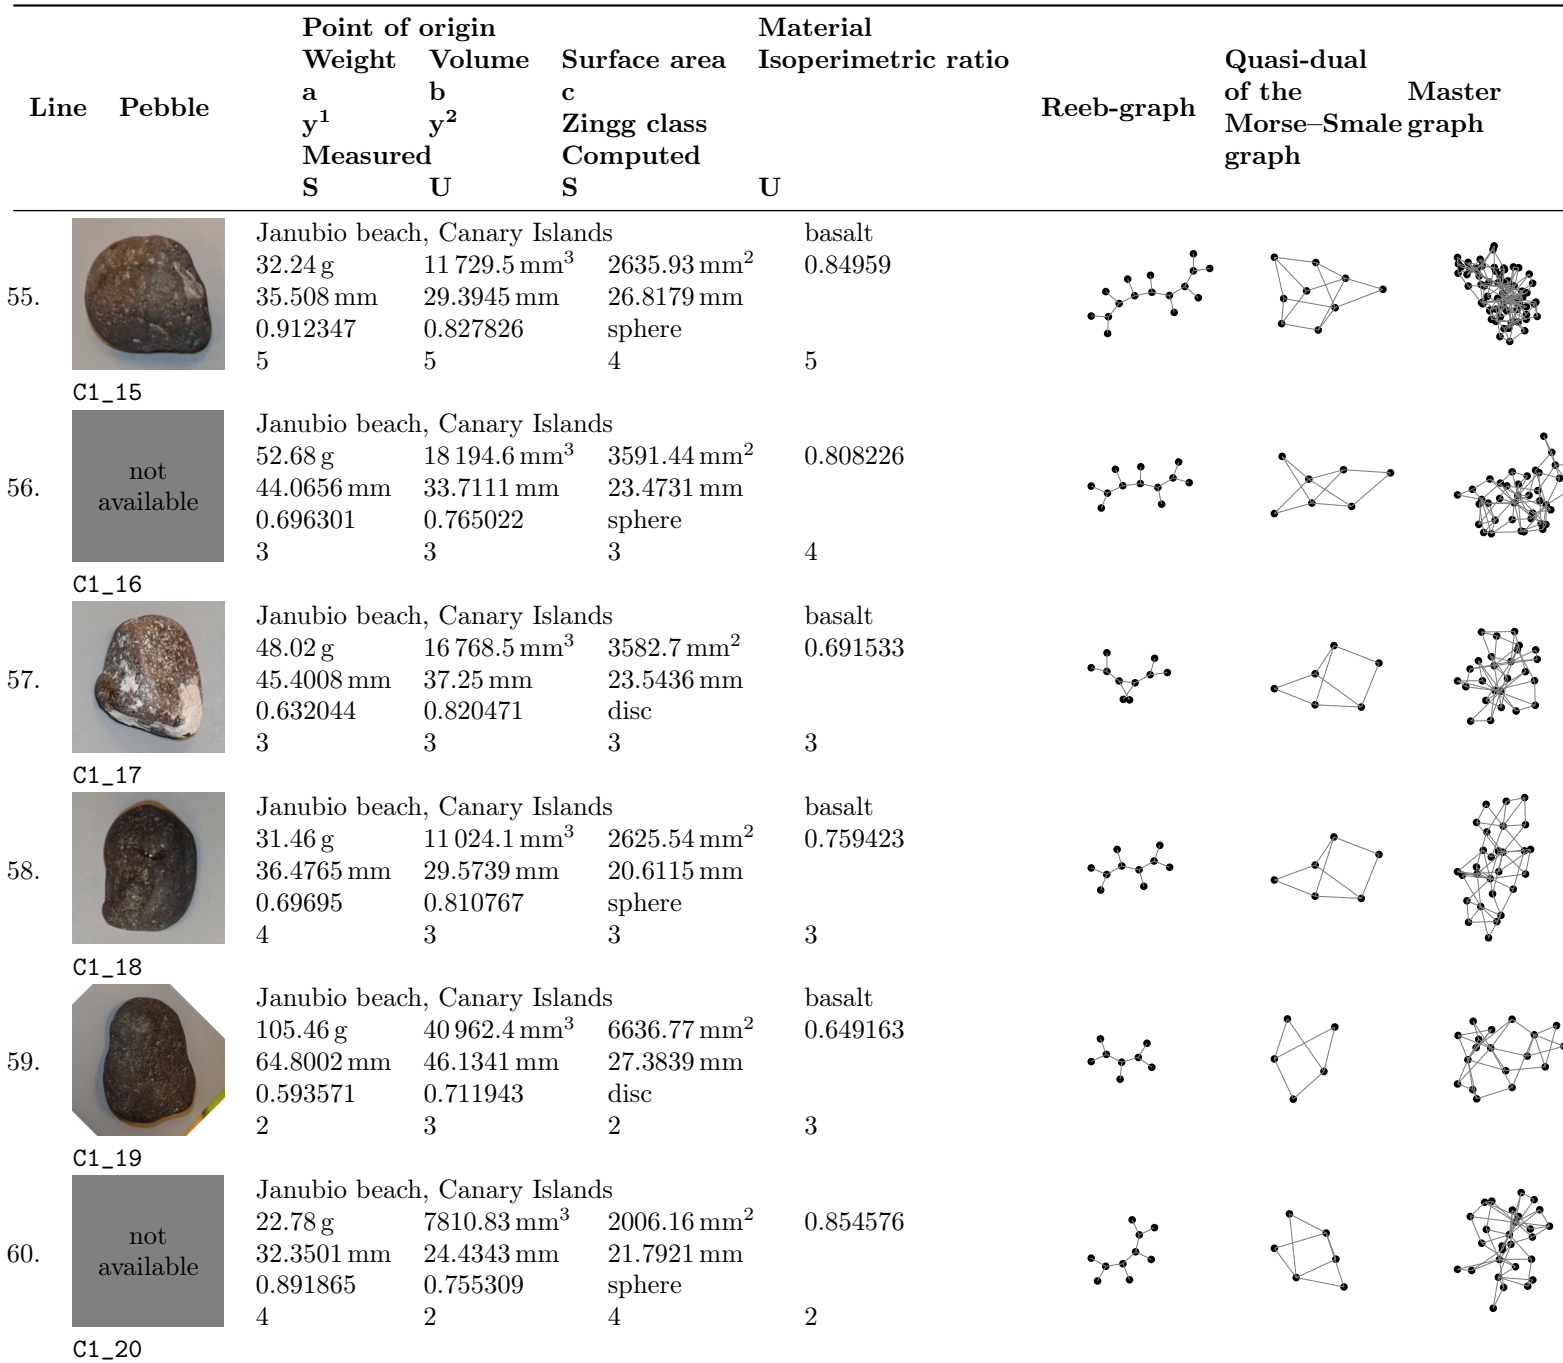   | 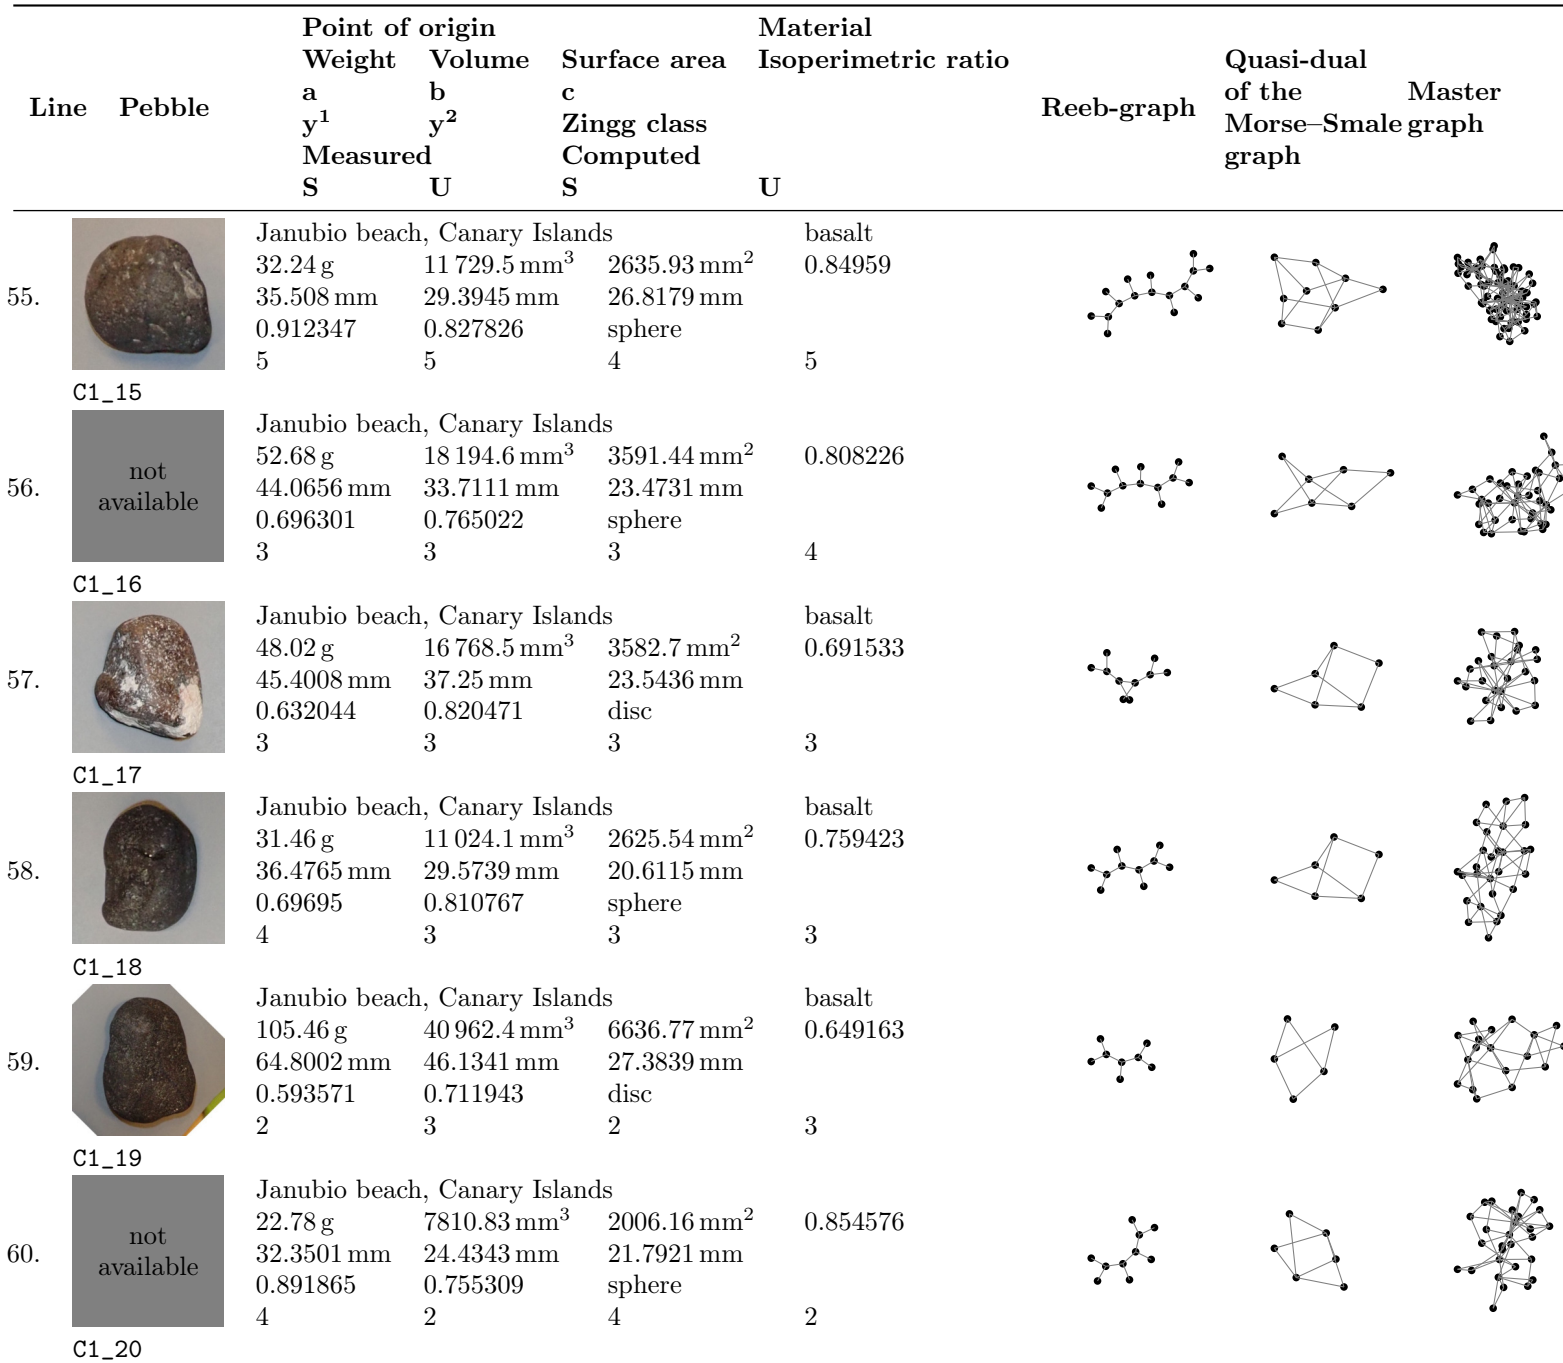   | 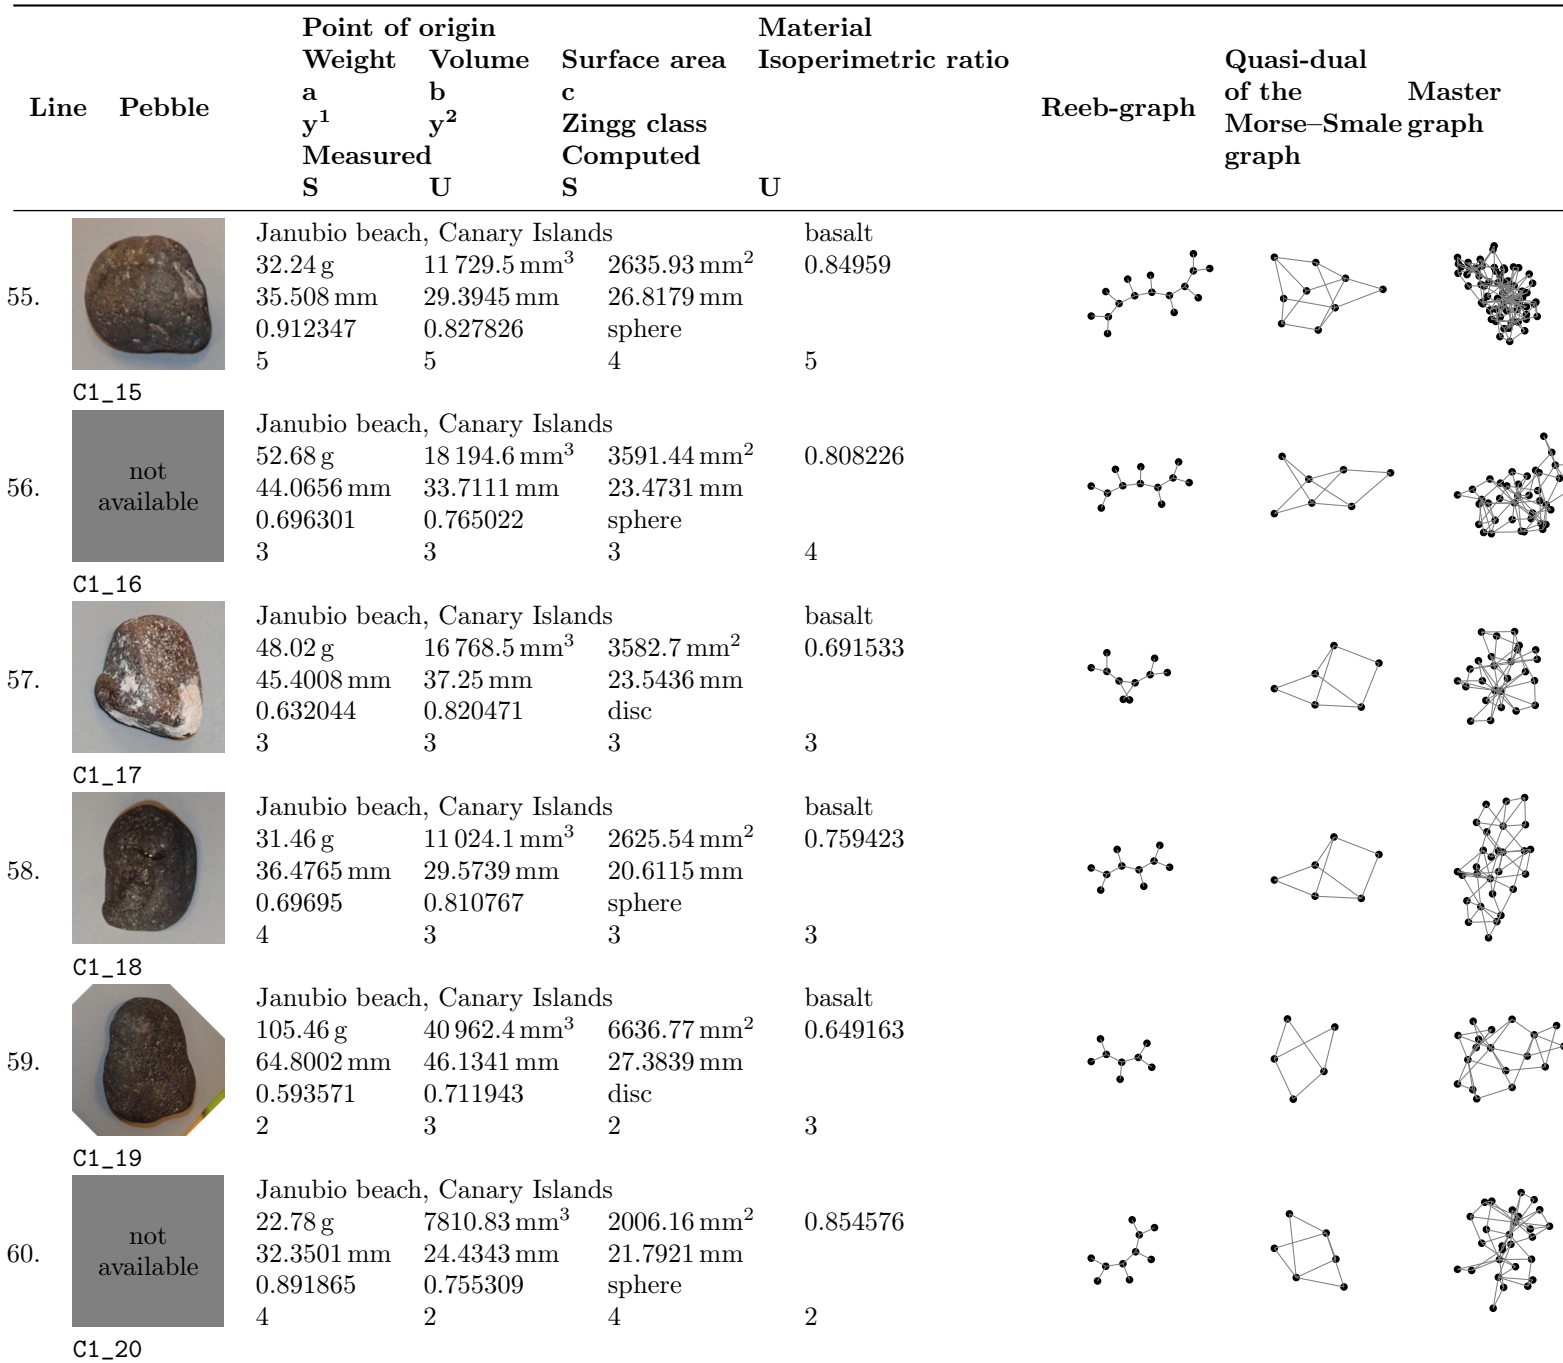   |                 |
|       | 52.68 g                                                                             | 18 194.6 mm <sup>3</sup>             | 3591.44 mm <sup>2</sup>  | 0.808226                          |          |                                                                                       |                                                                                       |                                                                                       |                 |
|       | 44.0656 mm                                                                          | 33.7111 mm                           | 23.4731 mm               |                                   |          |                                                                                       |                                                                                       |                                                                                       |                 |
|       | 0.696301                                                                            | 0.765022                             | sphere                   |                                   |          |                                                                                       |                                                                                       |                                                                                       |                 |
|       | 3                                                                                   | 3                                    | 3                        | 4                                 |          |                                                                                       |                                                                                       |                                                                                       |                 |
| C1_16 |                                                                                     |                                      |                          |                                   |          |                                                                                       |                                                                                       |                                                                                       |                 |
| 57.   | 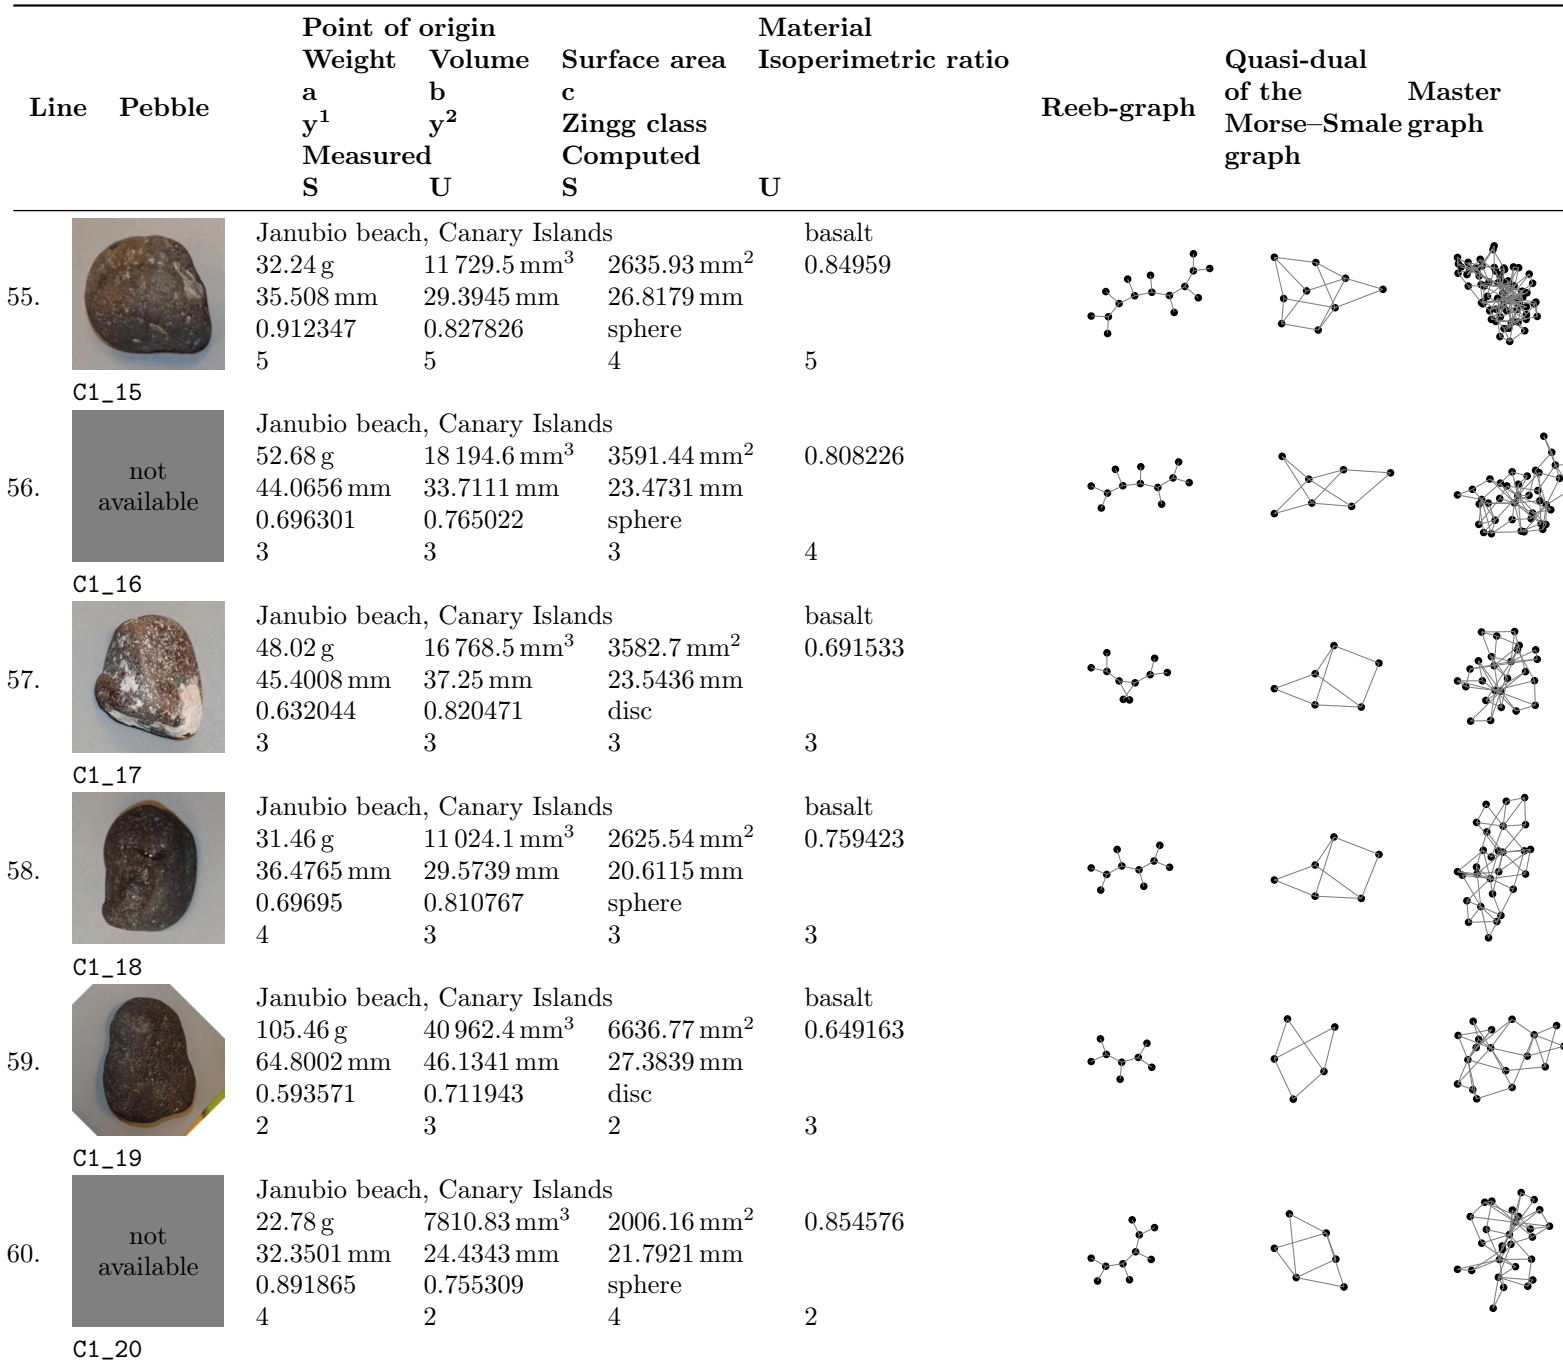   | Janubio beach, Canary Islands        |                          |                                   | basalt   | 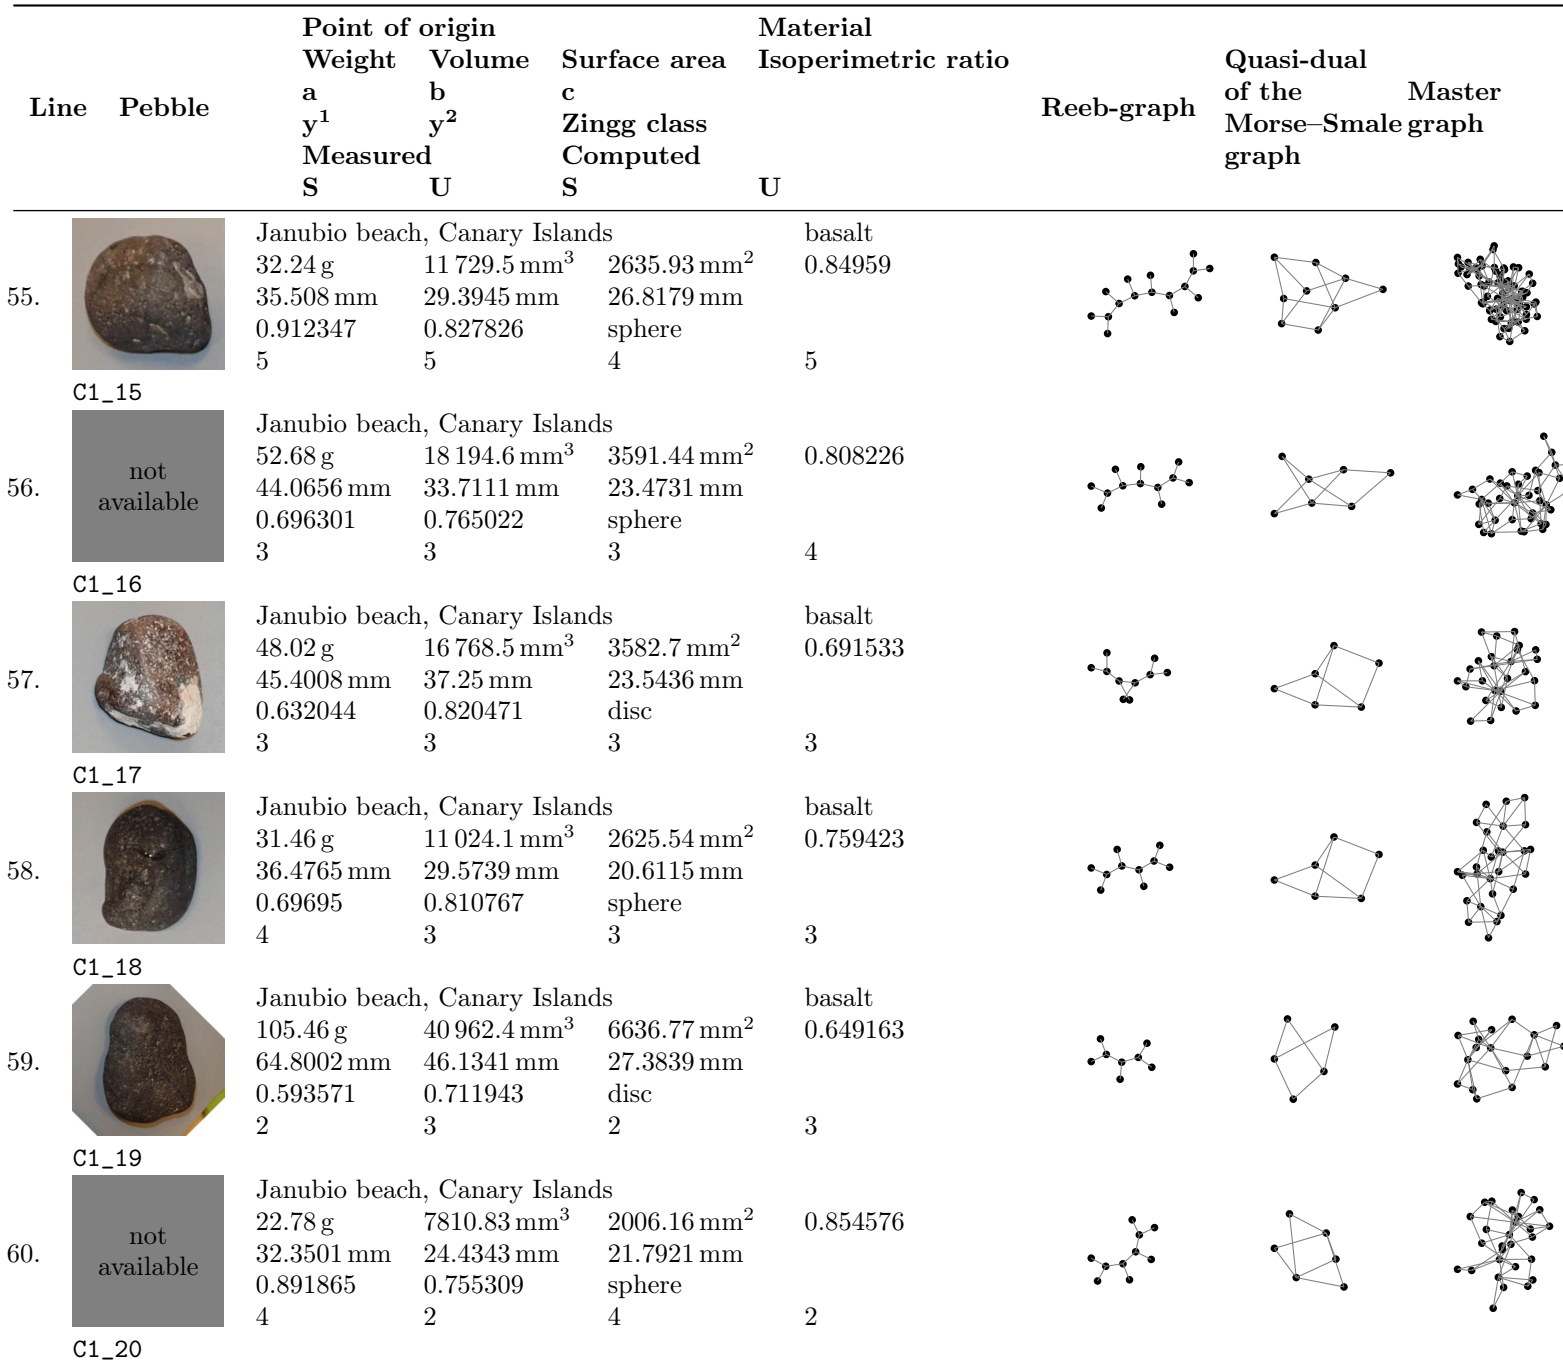   | 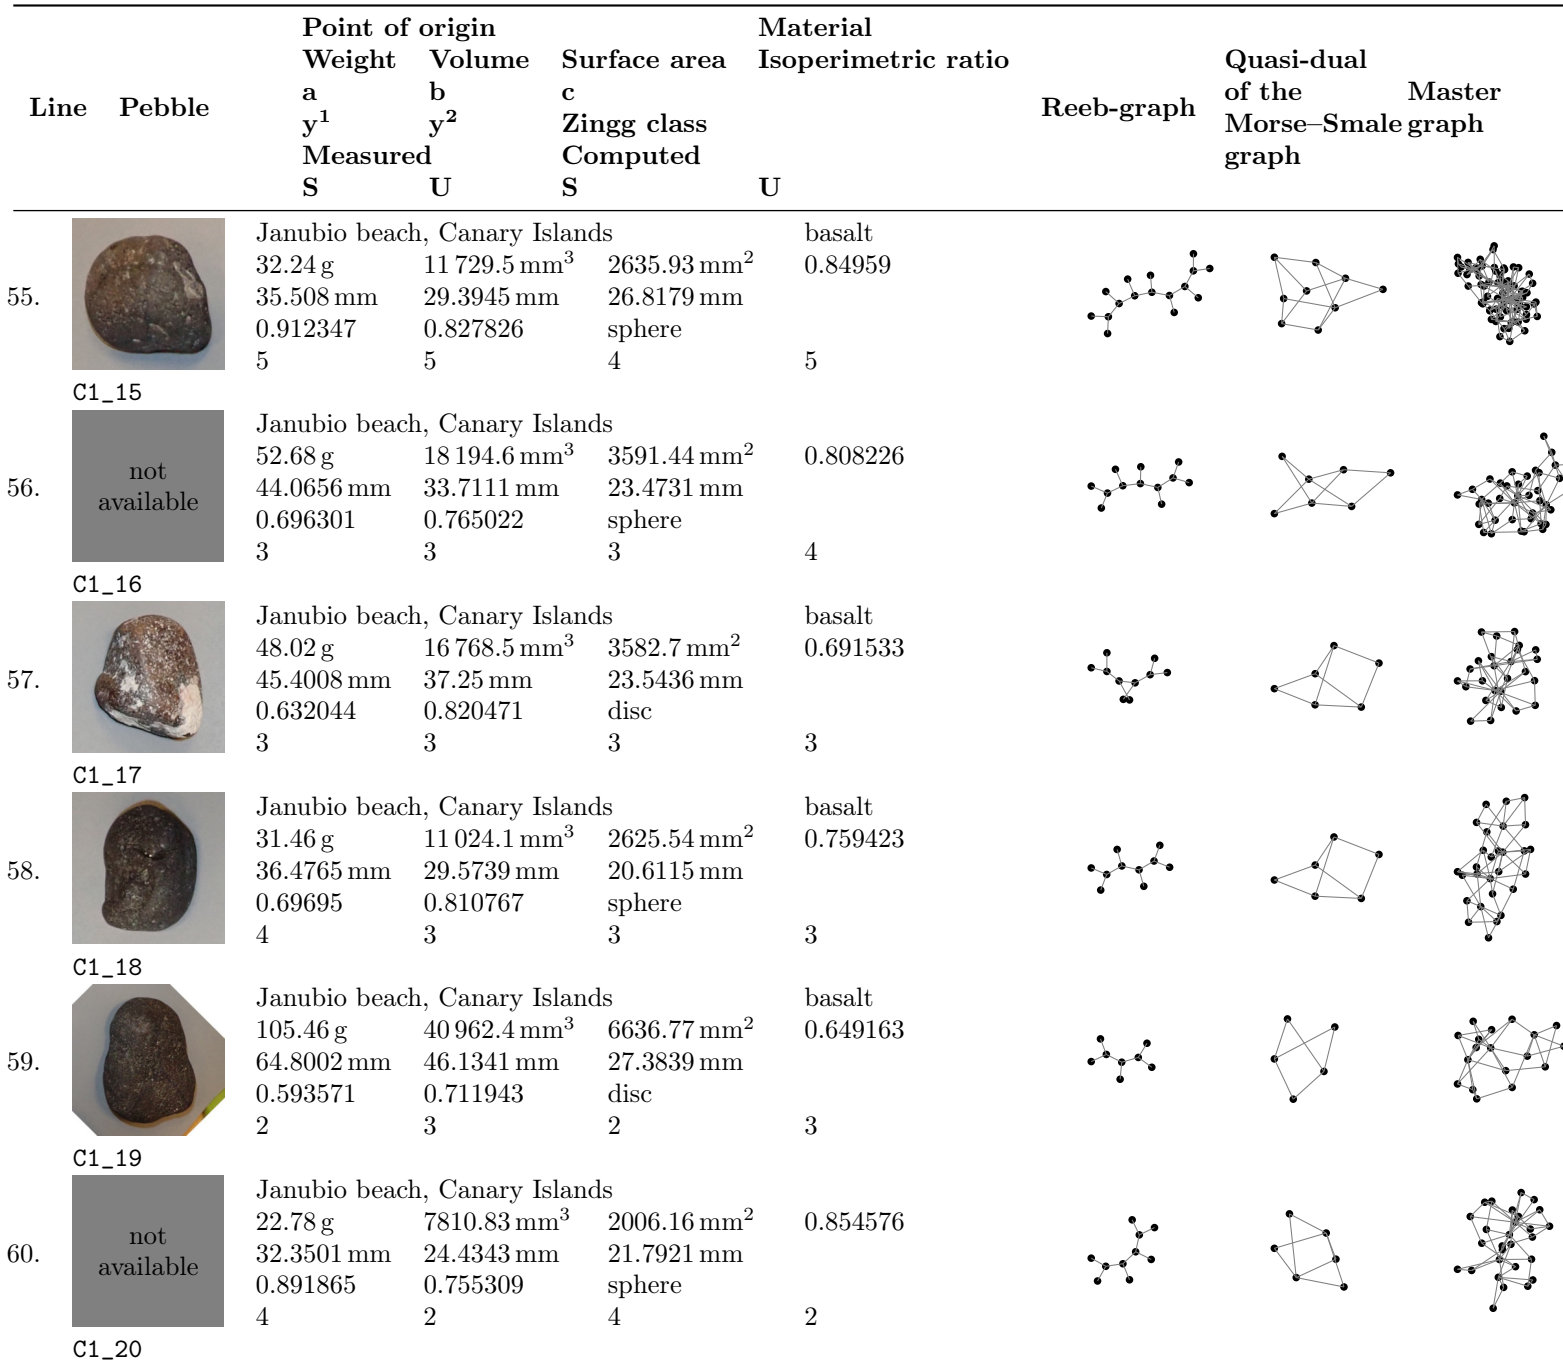   | 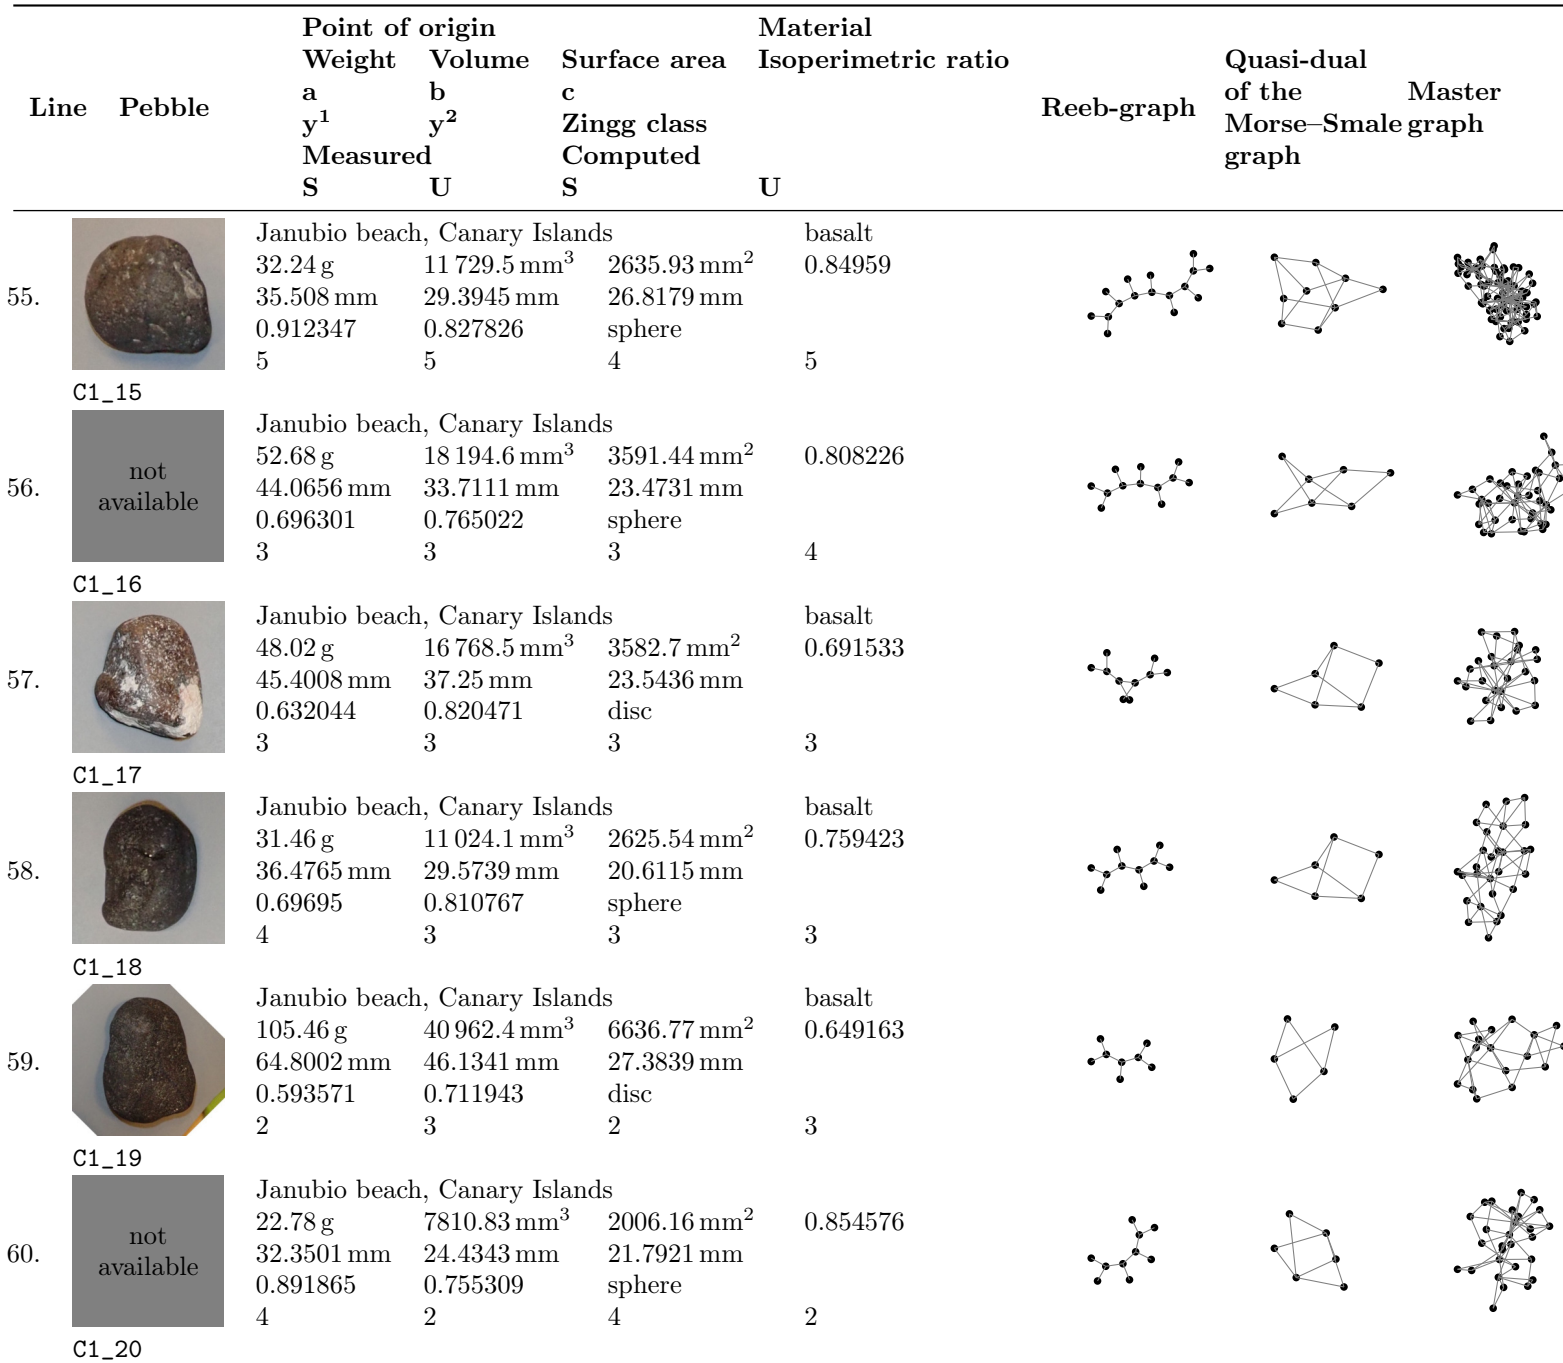   |                 |
|       | 48.02 g                                                                             | 16 768.5 mm <sup>3</sup>             | 3582.7 mm <sup>2</sup>   | 0.691533                          |          |                                                                                       |                                                                                       |                                                                                       |                 |
|       | 45.4008 mm                                                                          | 37.25 mm                             | 23.5436 mm               |                                   |          |                                                                                       |                                                                                       |                                                                                       |                 |
|       | 0.632044                                                                            | 0.820471                             | disc                     |                                   |          |                                                                                       |                                                                                       |                                                                                       |                 |
|       | 3                                                                                   | 3                                    | 3                        | 3                                 |          |                                                                                       |                                                                                       |                                                                                       |                 |
| C1_17 |                                                                                     |                                      |                          |                                   |          |                                                                                       |                                                                                       |                                                                                       |                 |
| 58.   | 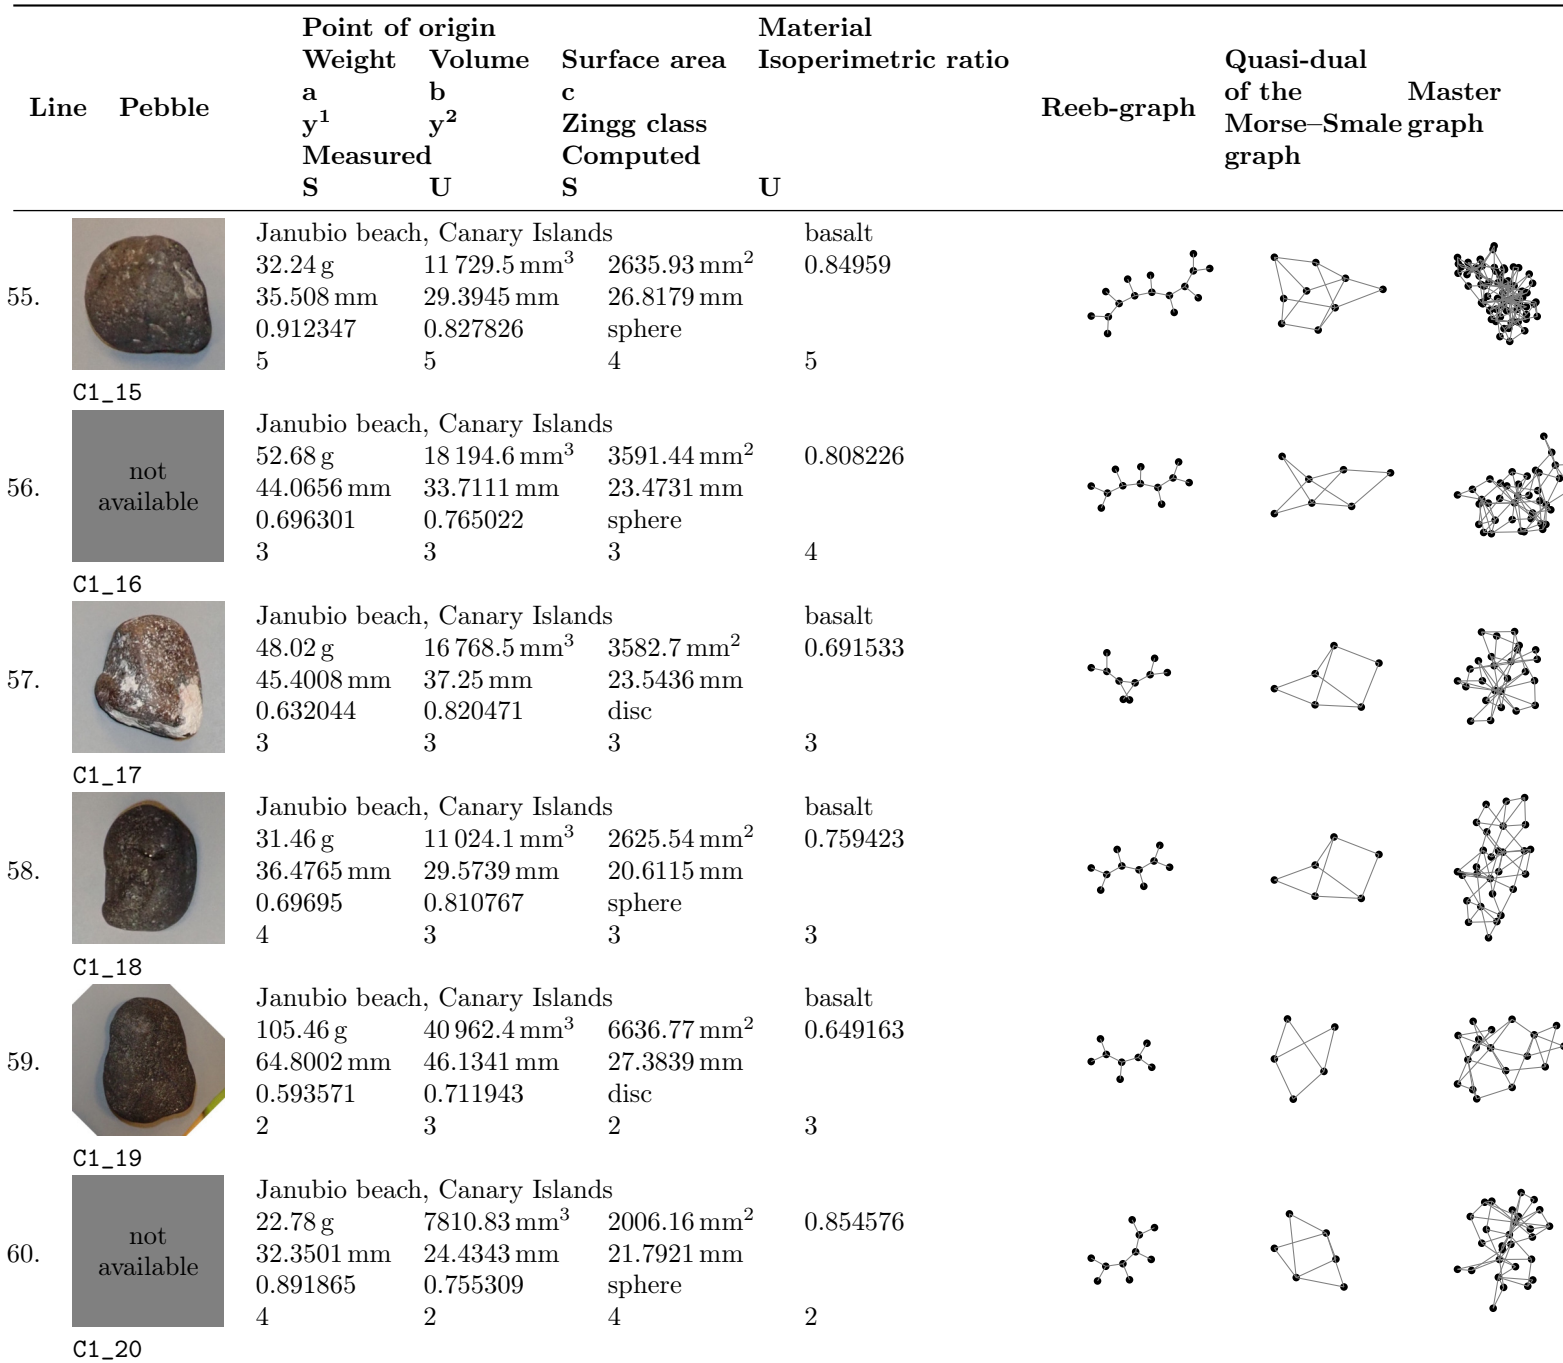  | Janubio beach, Canary Islands        |                          |                                   | basalt   | 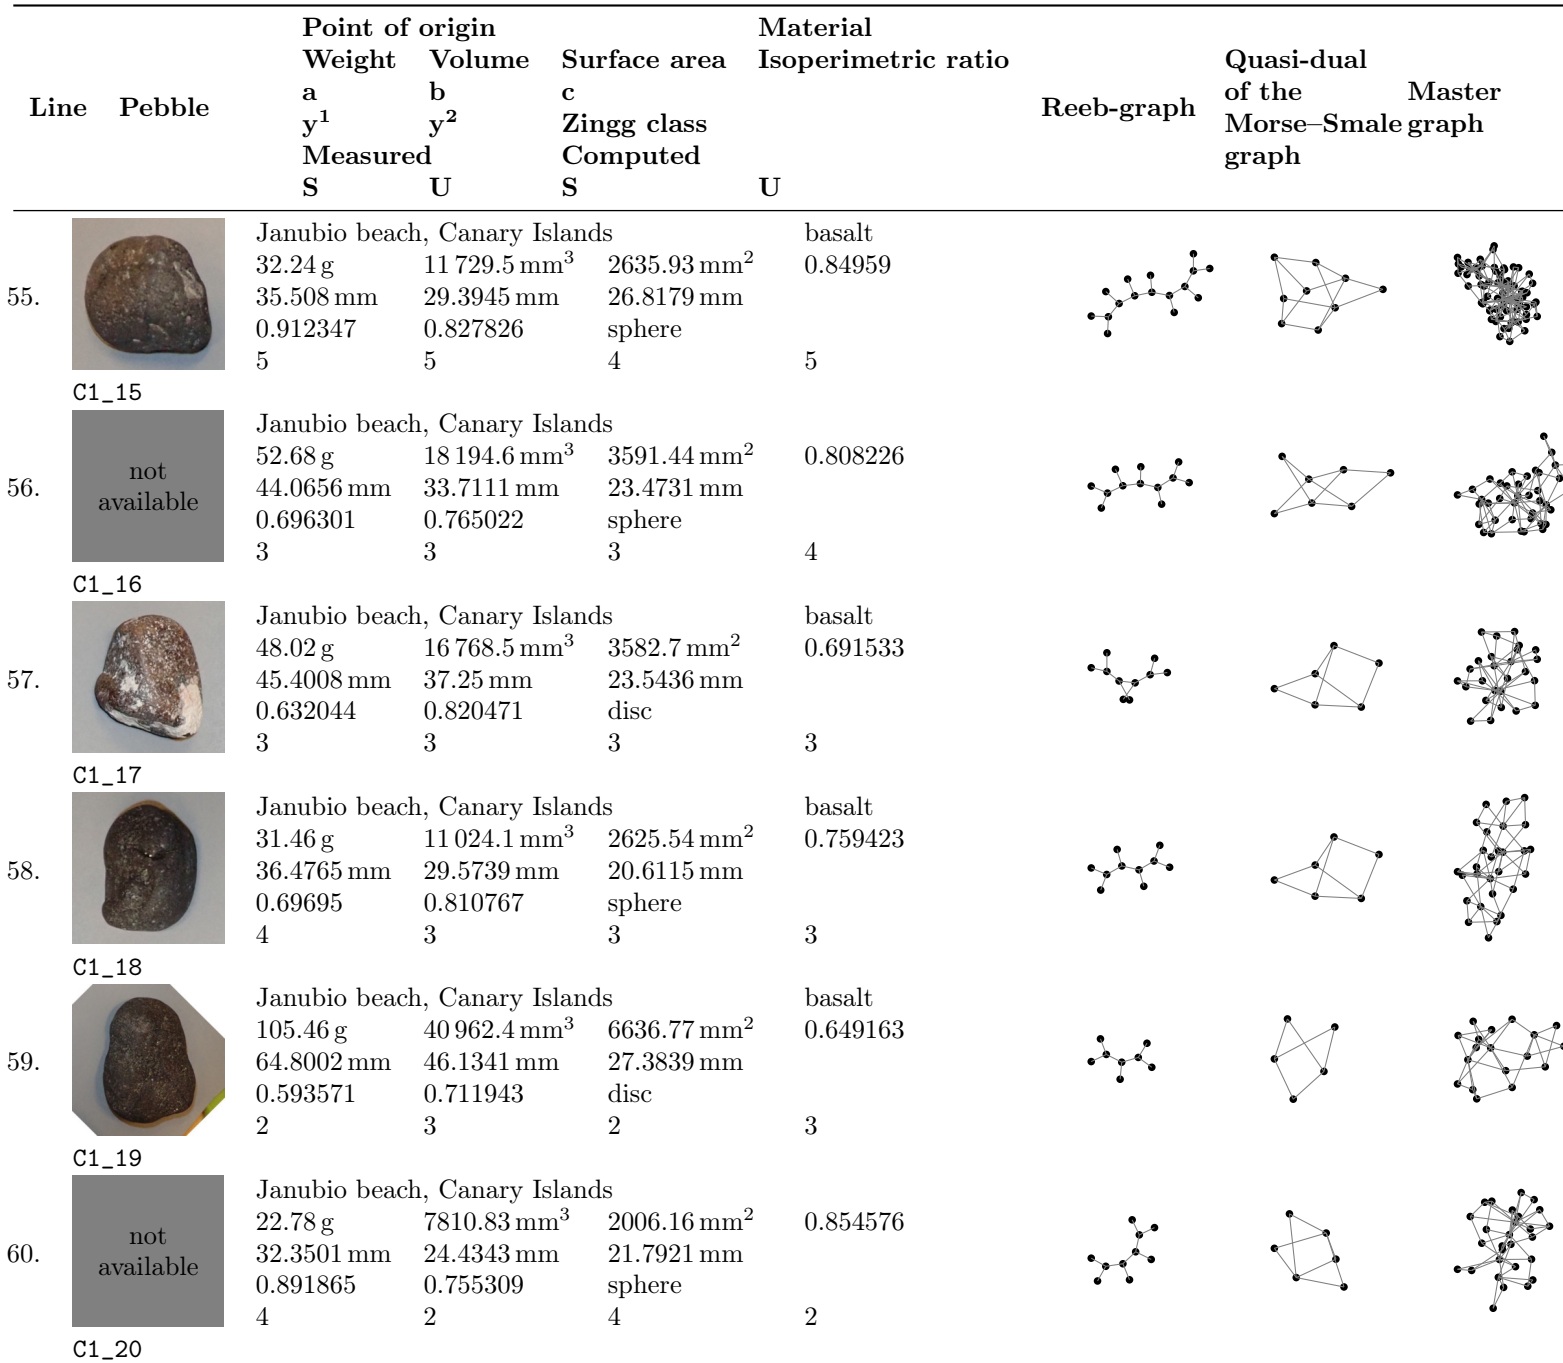  | 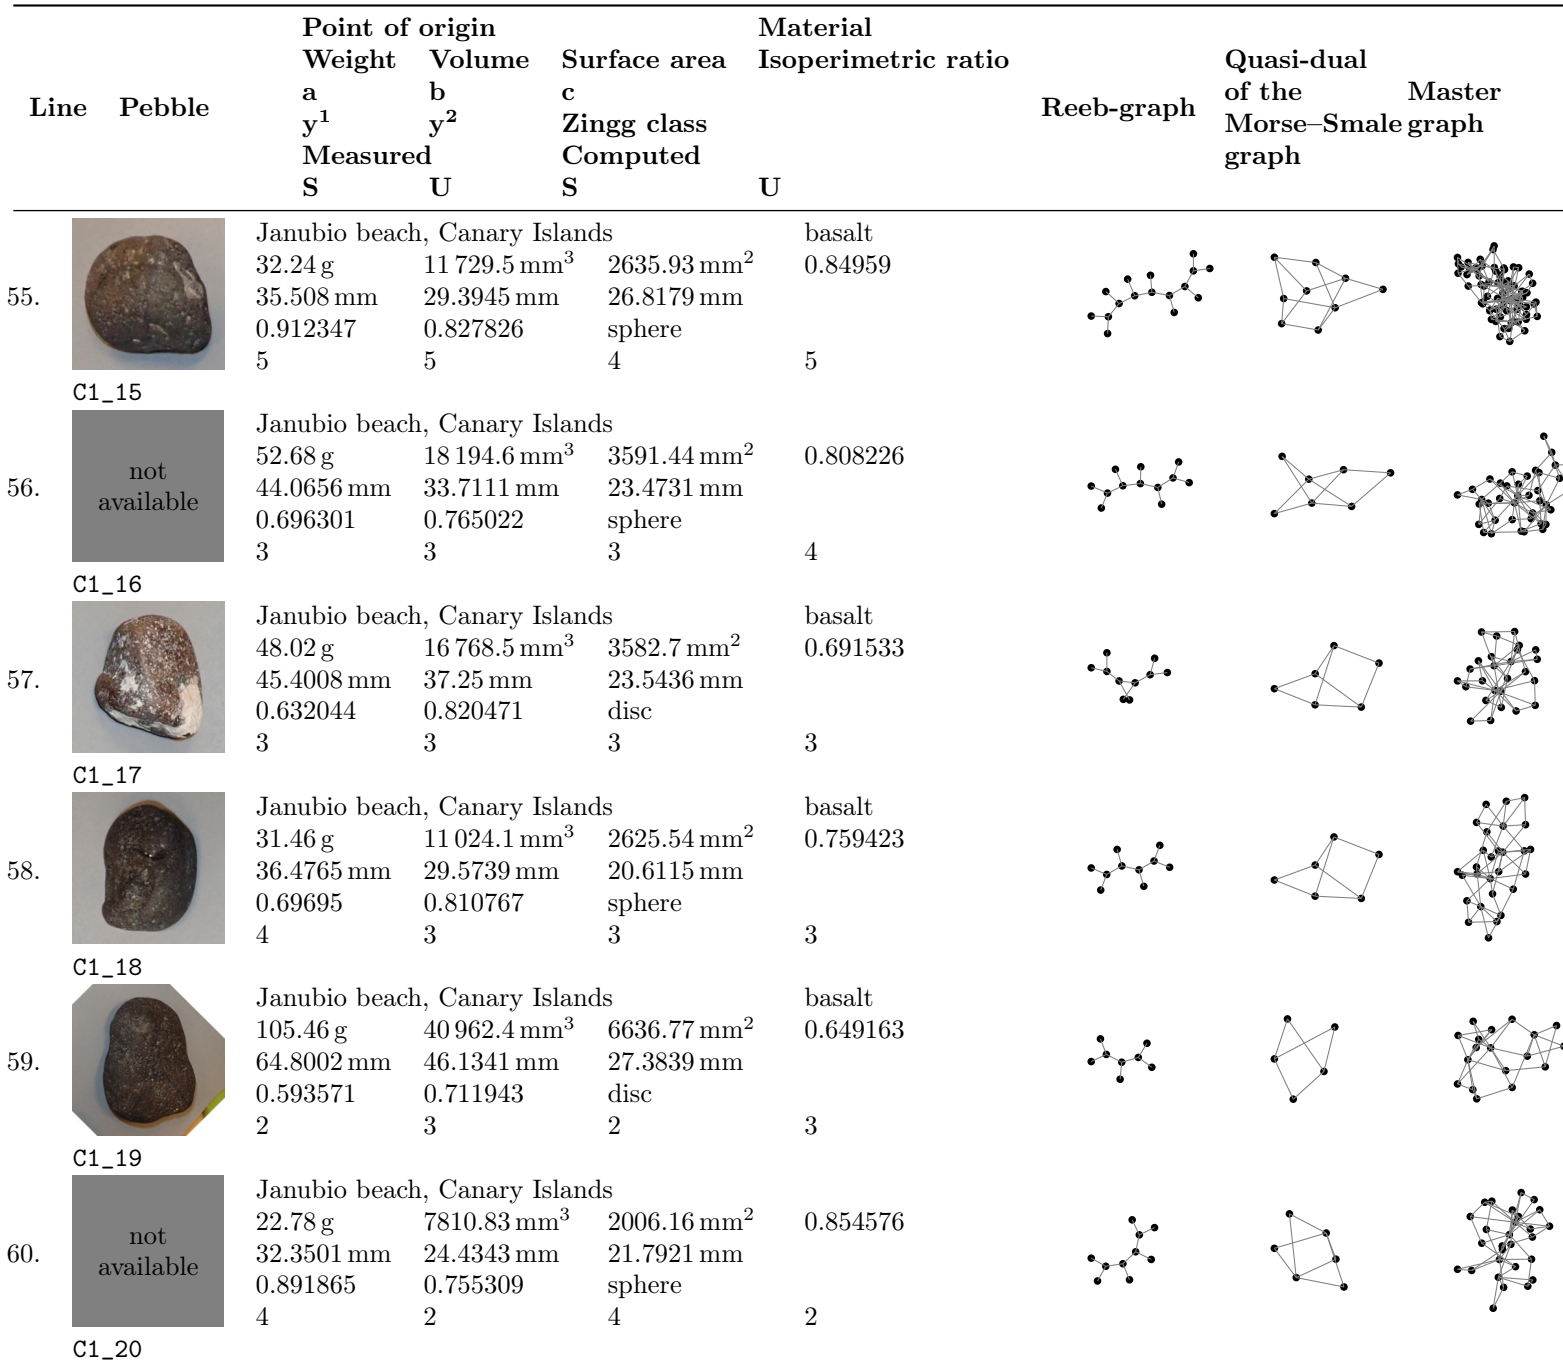  | 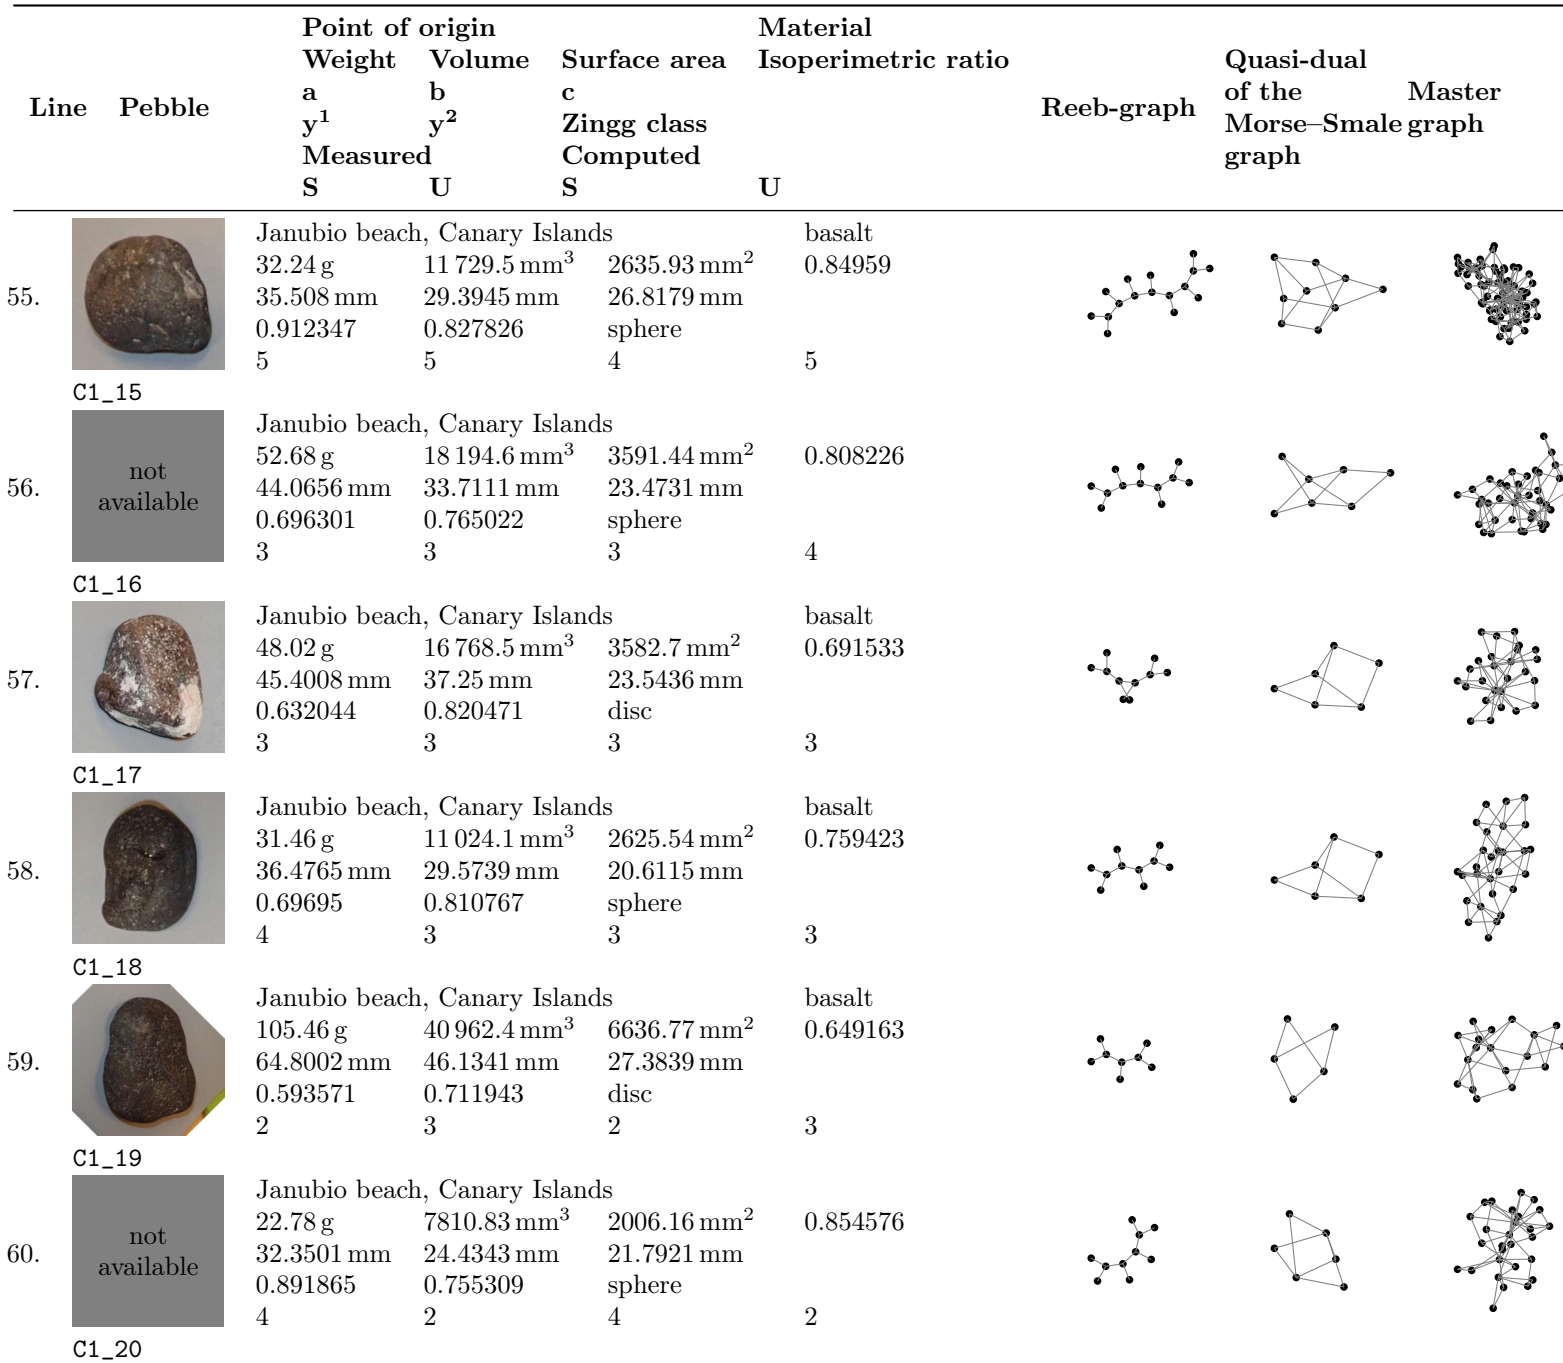  |                 |
|       | 31.46 g                                                                             | 11 024.1 mm <sup>3</sup>             | 2625.54 mm <sup>2</sup>  | 0.759423                          |          |                                                                                       |                                                                                       |                                                                                       |                 |
|       | 36.4765 mm                                                                          | 29.5739 mm                           | 20.6115 mm               |                                   |          |                                                                                       |                                                                                       |                                                                                       |                 |
|       | 0.69695                                                                             | 0.810767                             | sphere                   |                                   |          |                                                                                       |                                                                                       |                                                                                       |                 |
|       | 4                                                                                   | 3                                    | 3                        | 3                                 |          |                                                                                       |                                                                                       |                                                                                       |                 |
| C1_18 |                                                                                     |                                      |                          |                                   |          |                                                                                       |                                                                                       |                                                                                       |                 |
| 59.   | 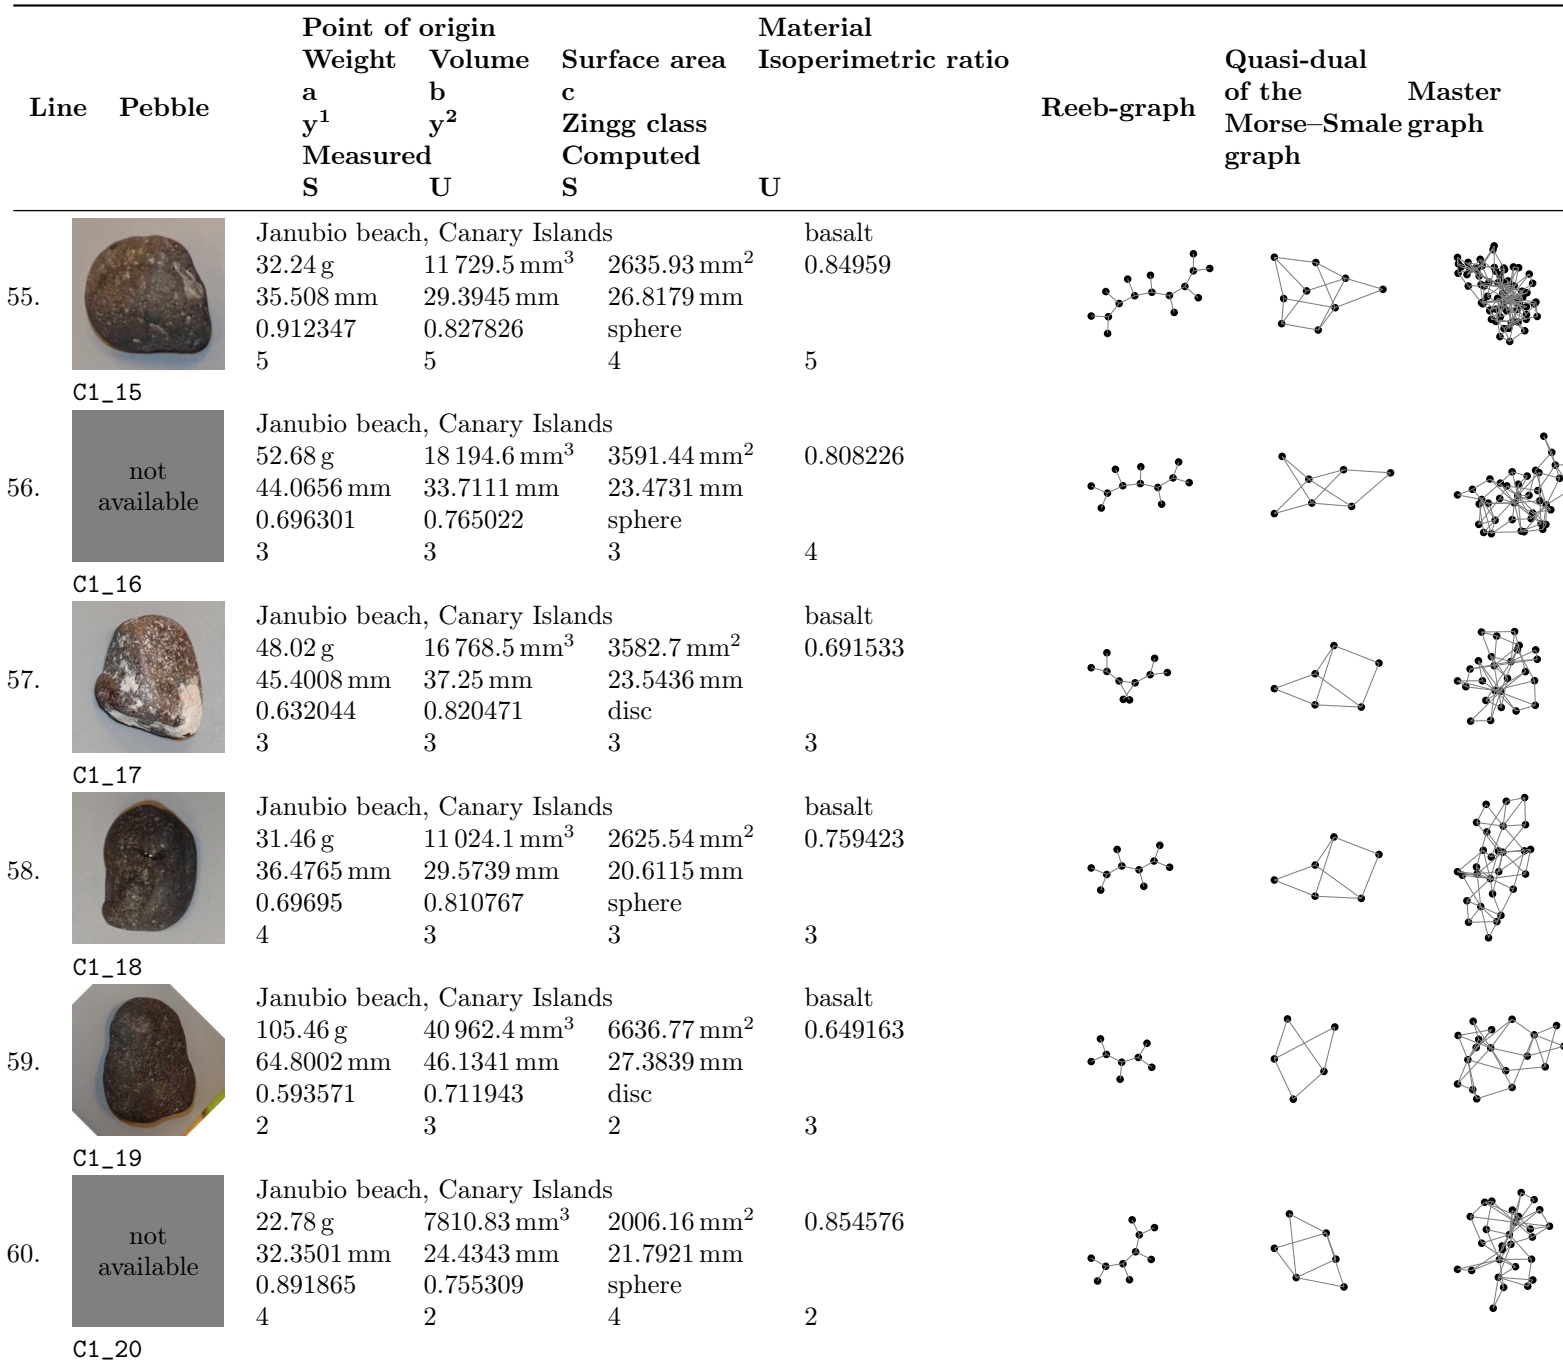 | Janubio beach, Canary Islands        |                          |                                   | basalt   | 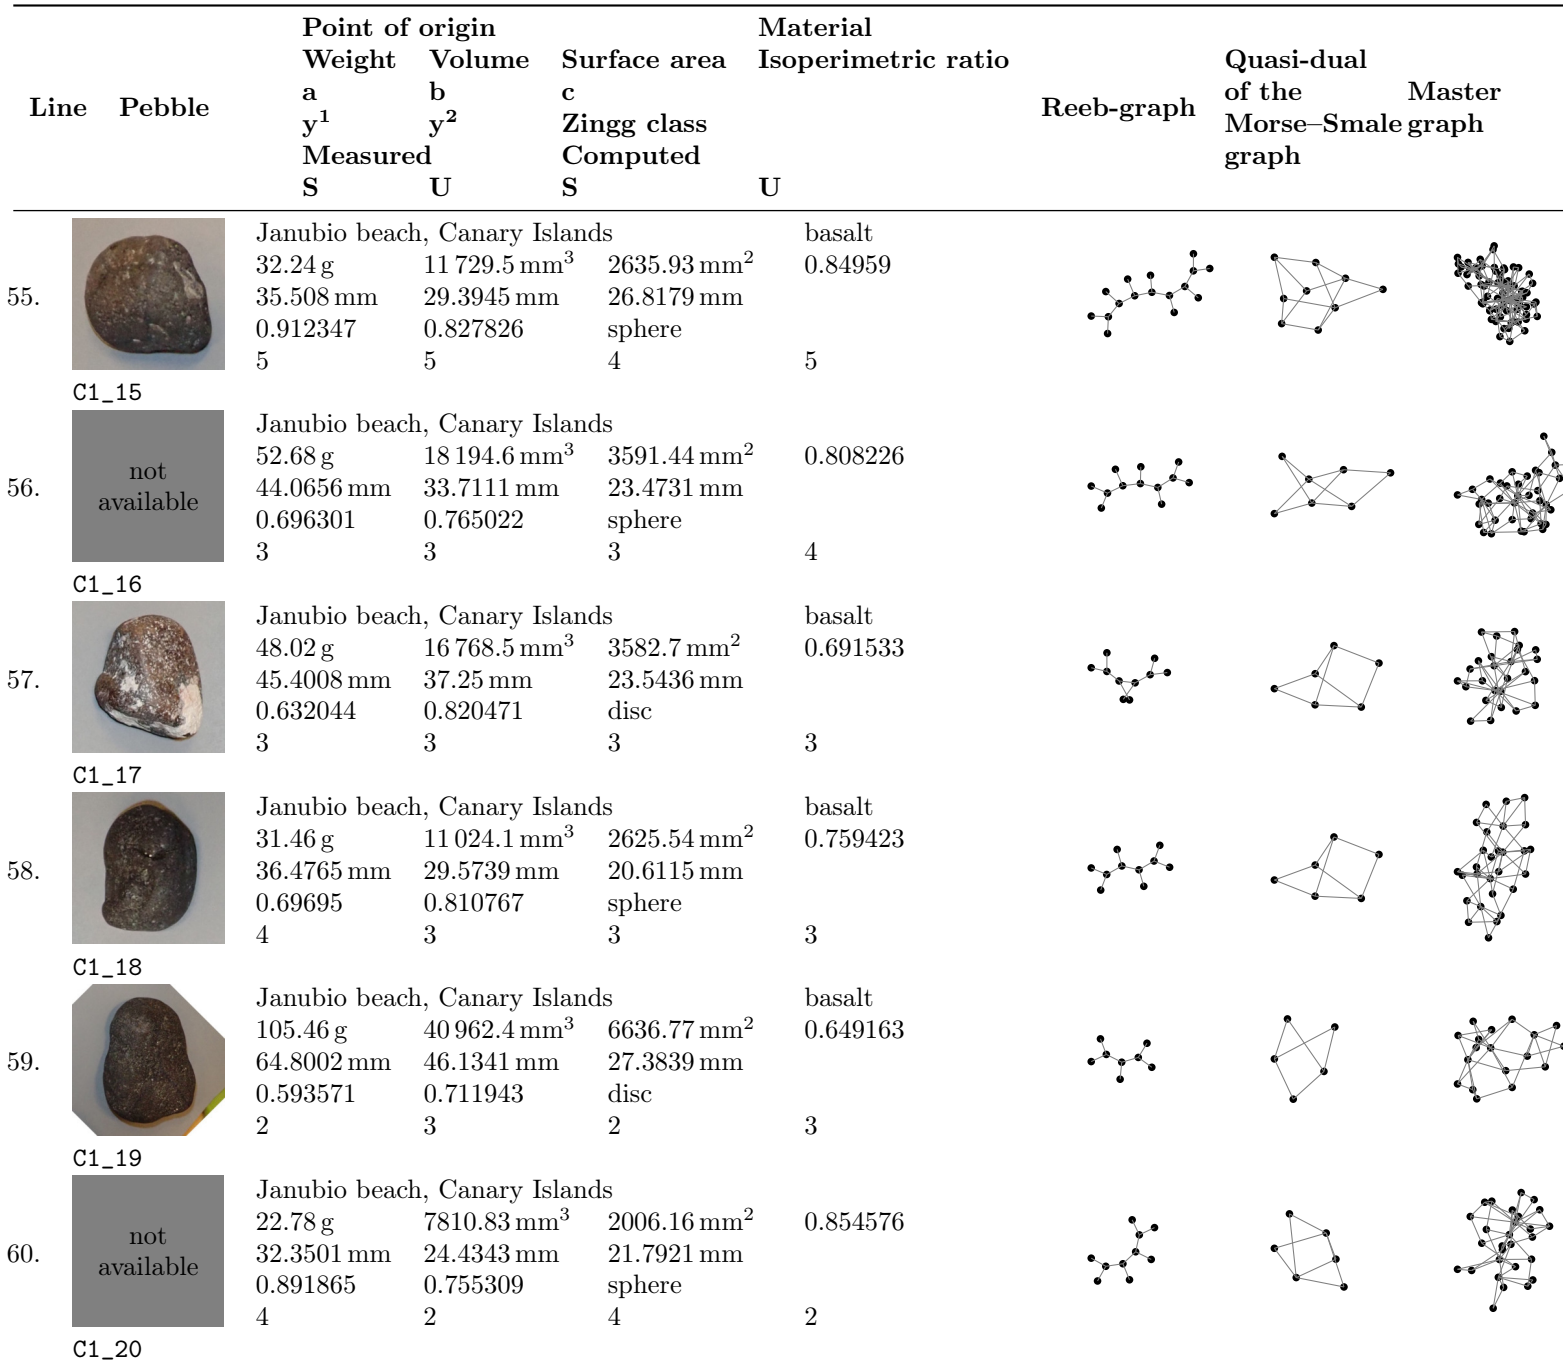 | 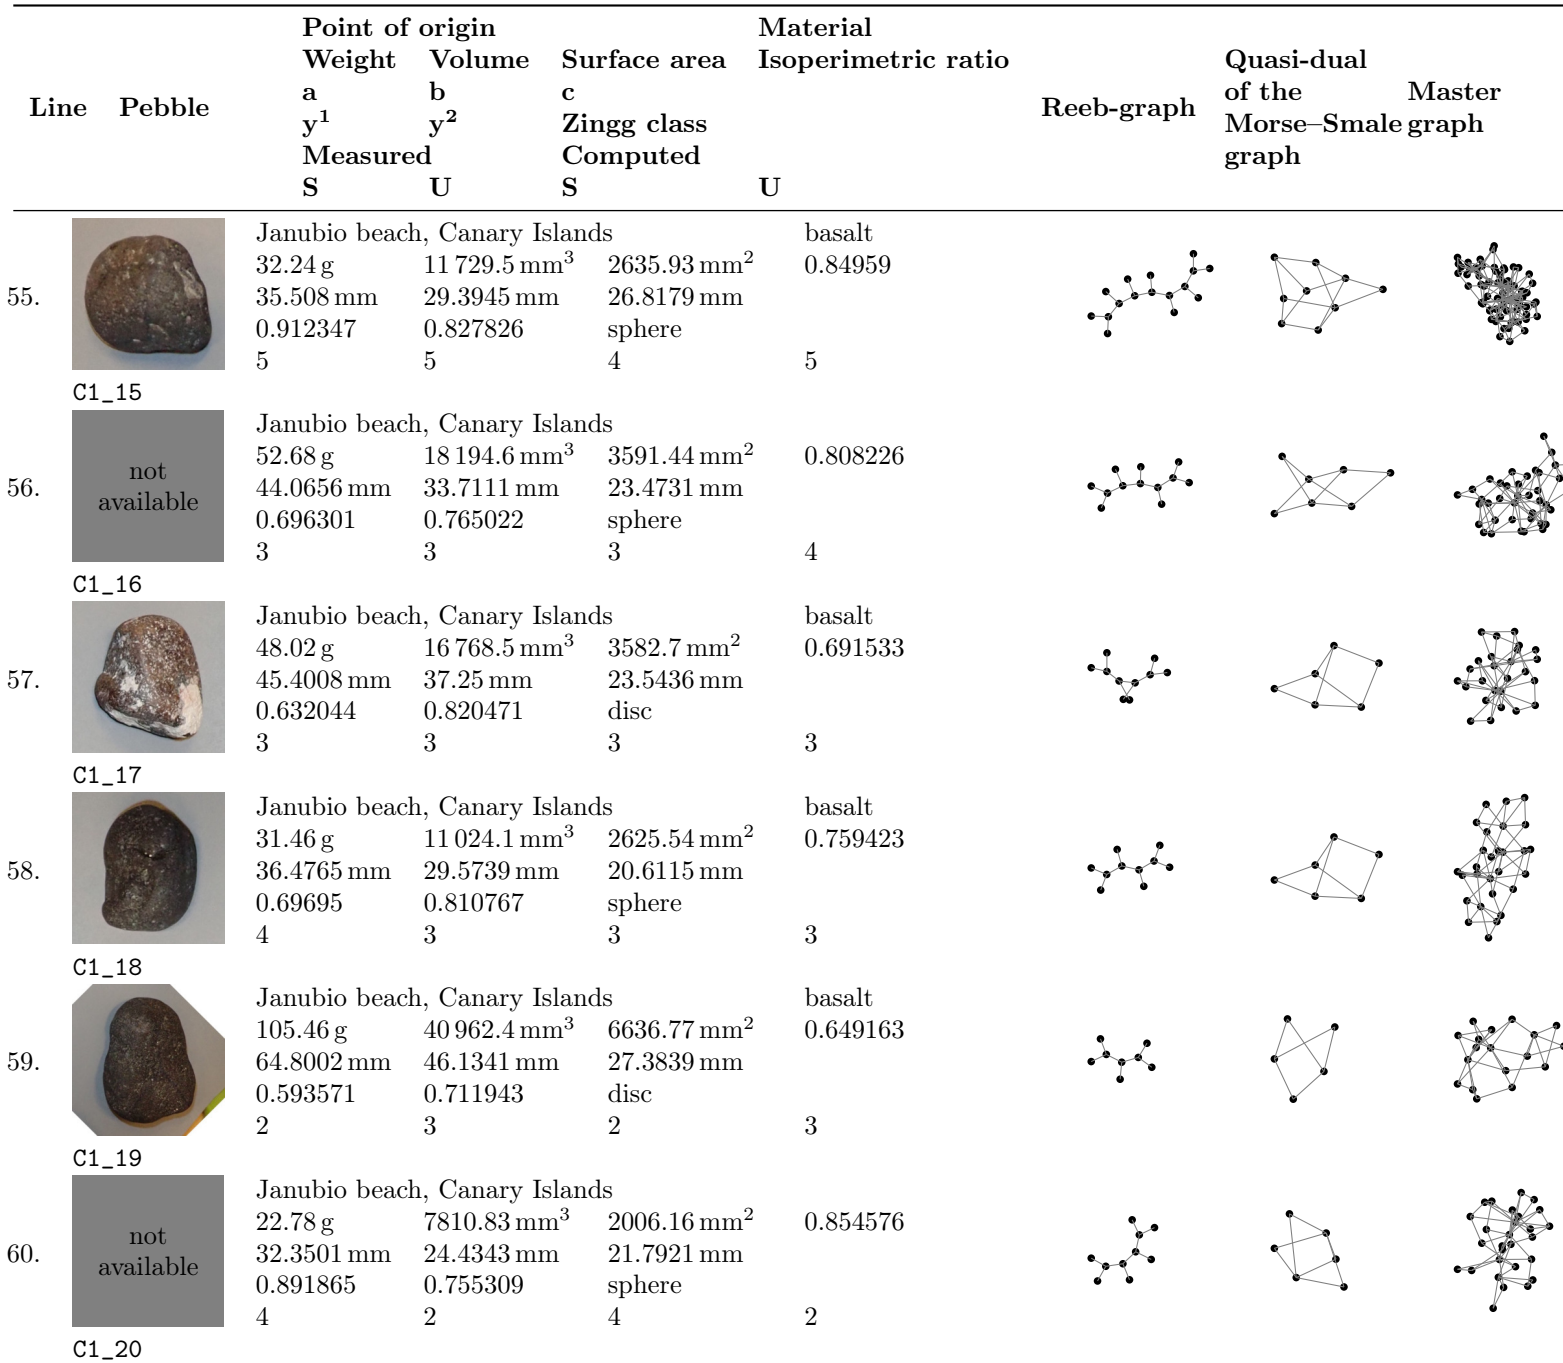 | 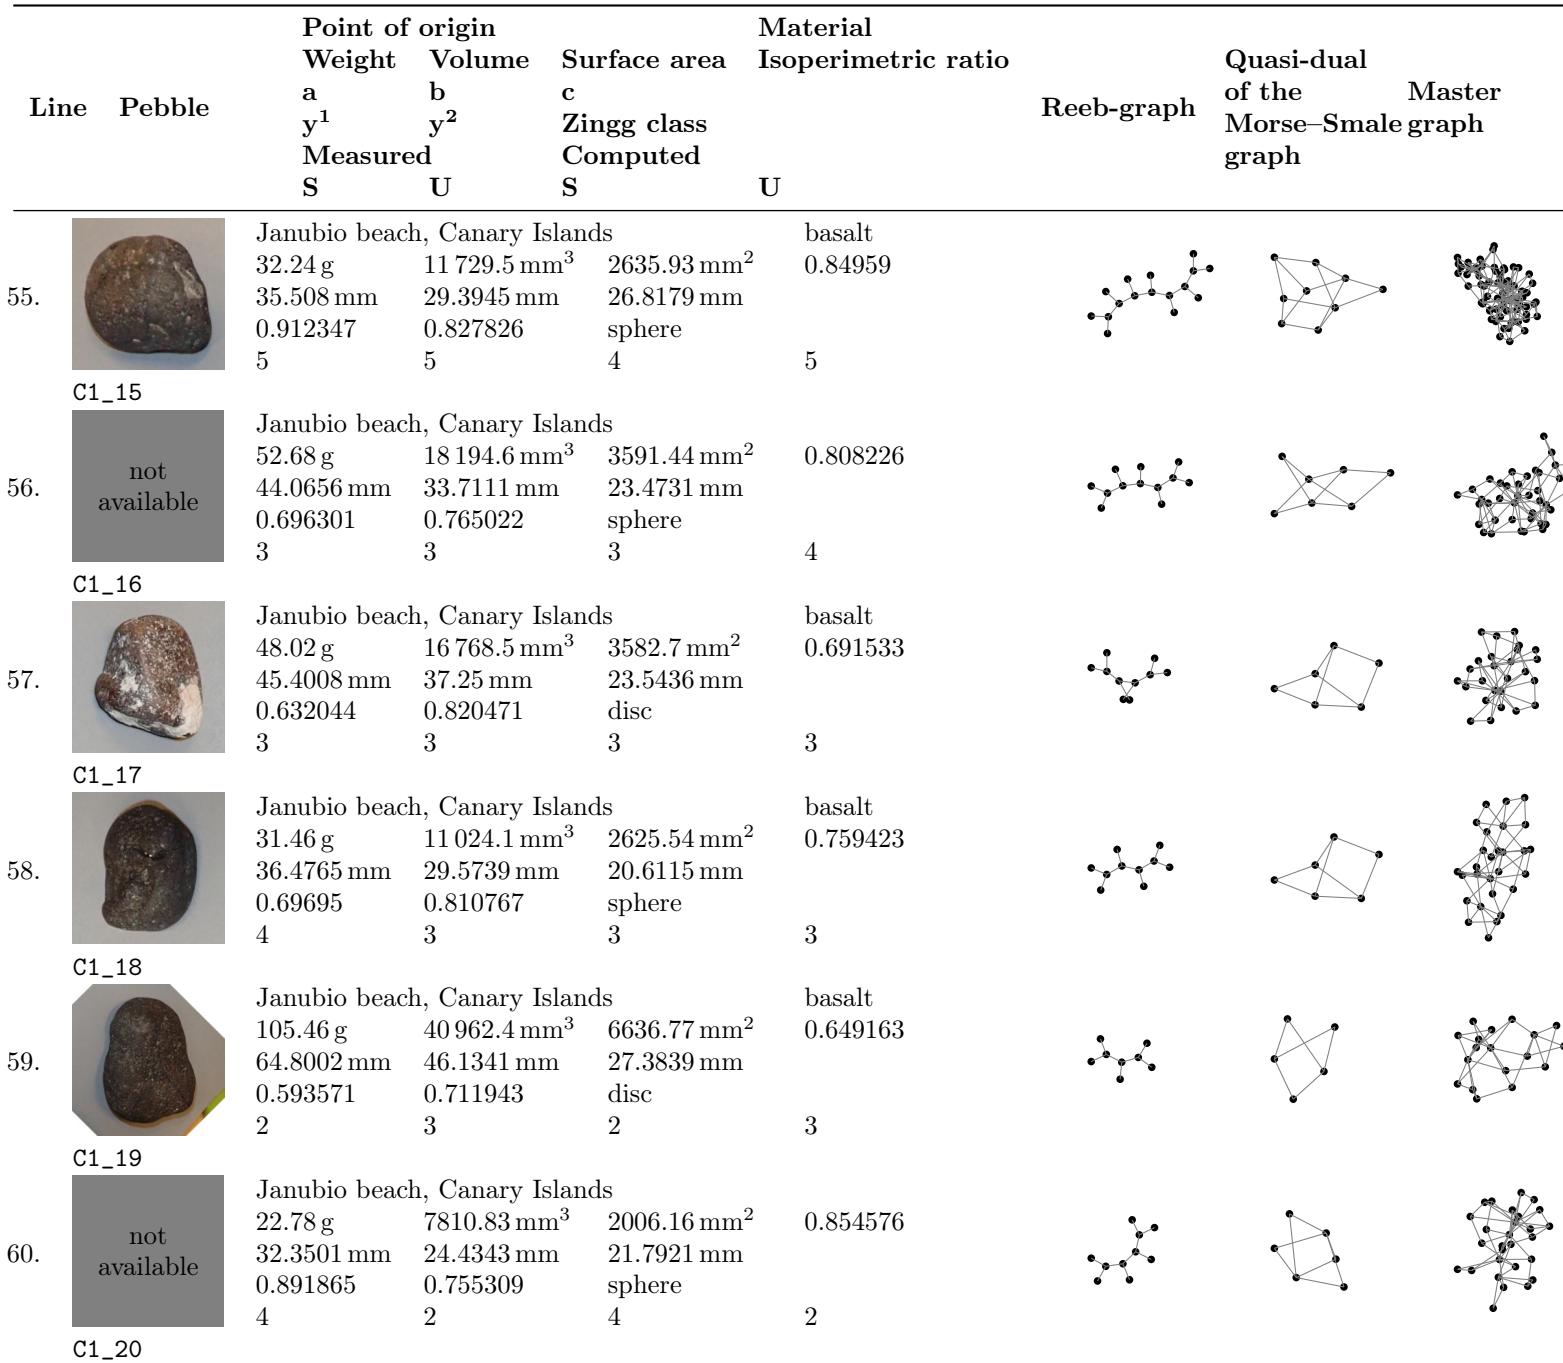 |                 |
|       | 105.46 g                                                                            | 40 962.4 mm <sup>3</sup>             | 6636.77 mm <sup>2</sup>  | 0.649163                          |          |                                                                                       |                                                                                       |                                                                                       |                 |
|       | 64.8002 mm                                                                          | 46.1341 mm                           | 27.3839 mm               |                                   |          |                                                                                       |                                                                                       |                                                                                       |                 |
|       | 0.593571                                                                            | 0.711943                             | disc                     |                                   |          |                                                                                       |                                                                                       |                                                                                       |                 |
|       | 2                                                                                   | 3                                    | 2                        | 3                                 |          |                                                                                       |                                                                                       |                                                                                       |                 |
| C1_19 |                                                                                     |                                      |                          |                                   |          |                                                                                       |                                                                                       |                                                                                       |                 |
| 60.   | 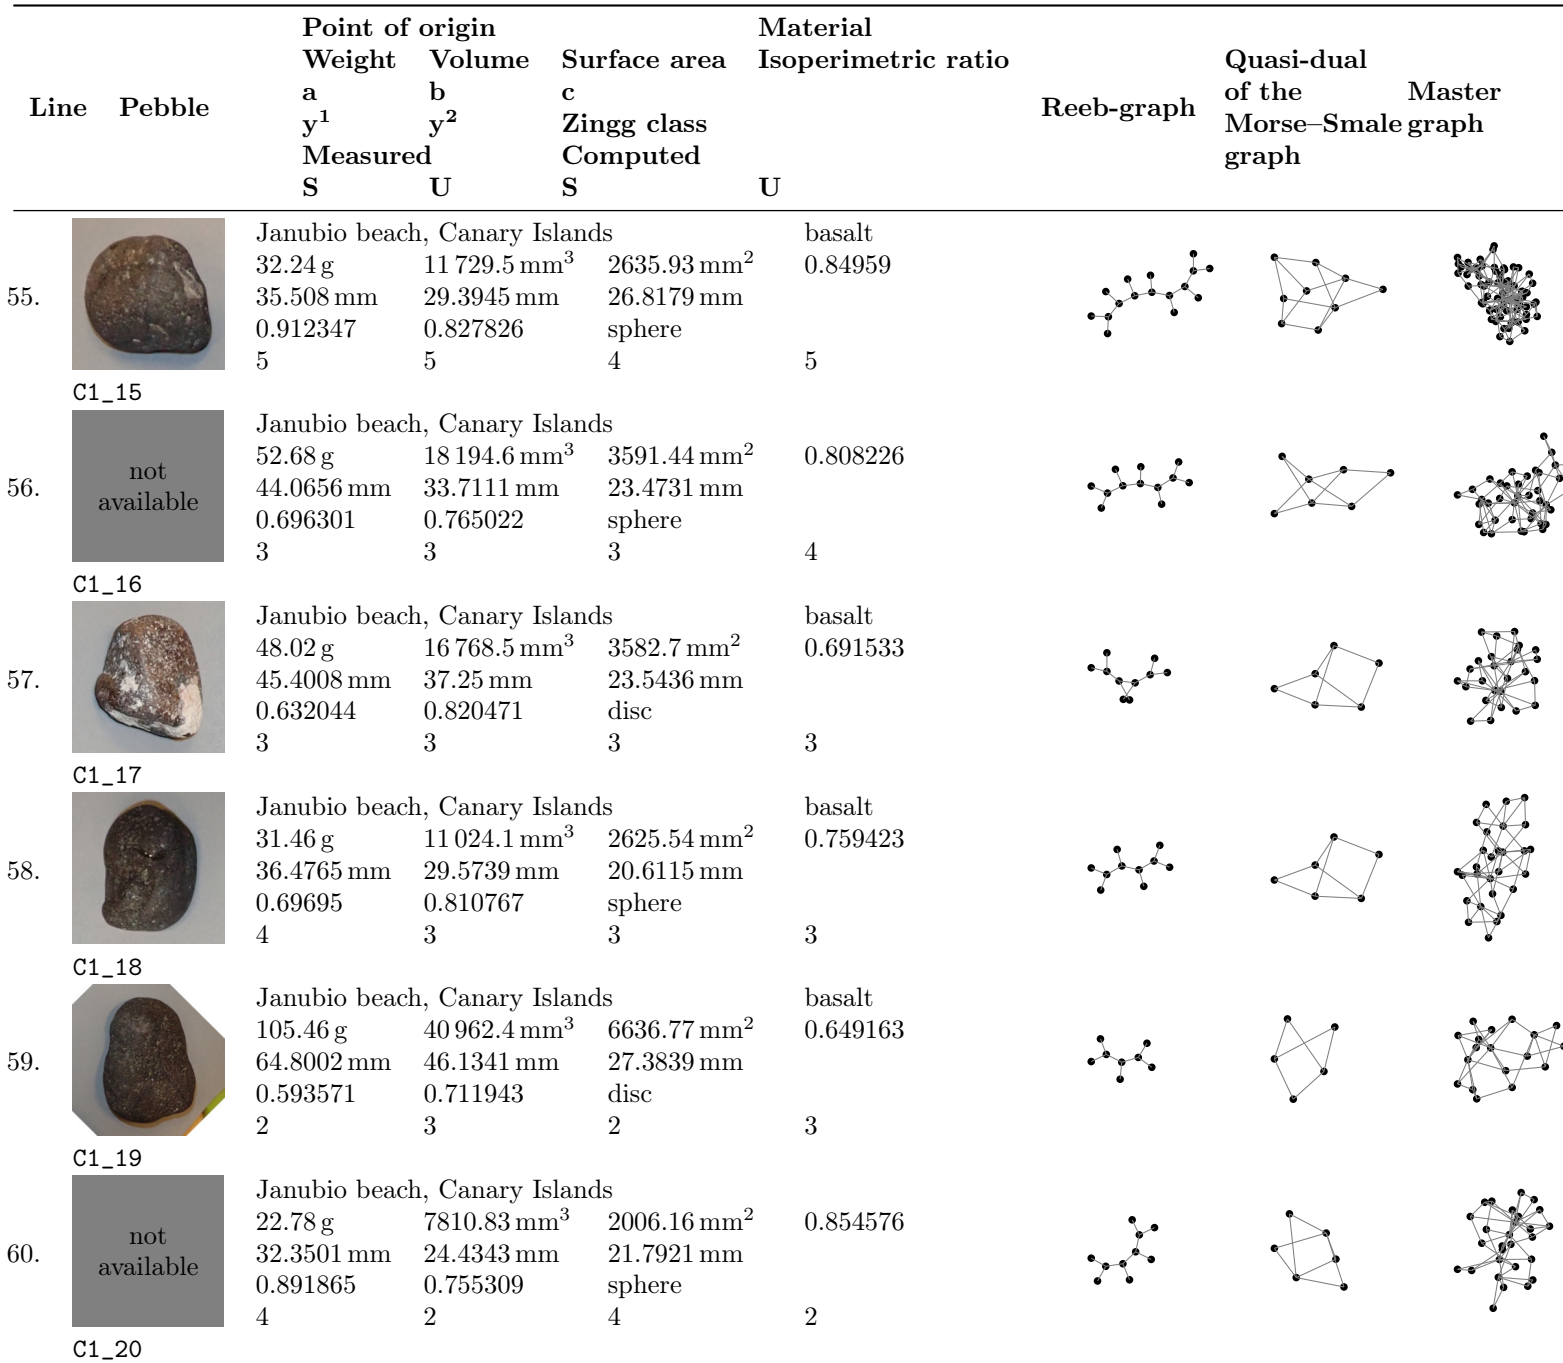 | Janubio beach, Canary Islands        |                          |                                   |          | 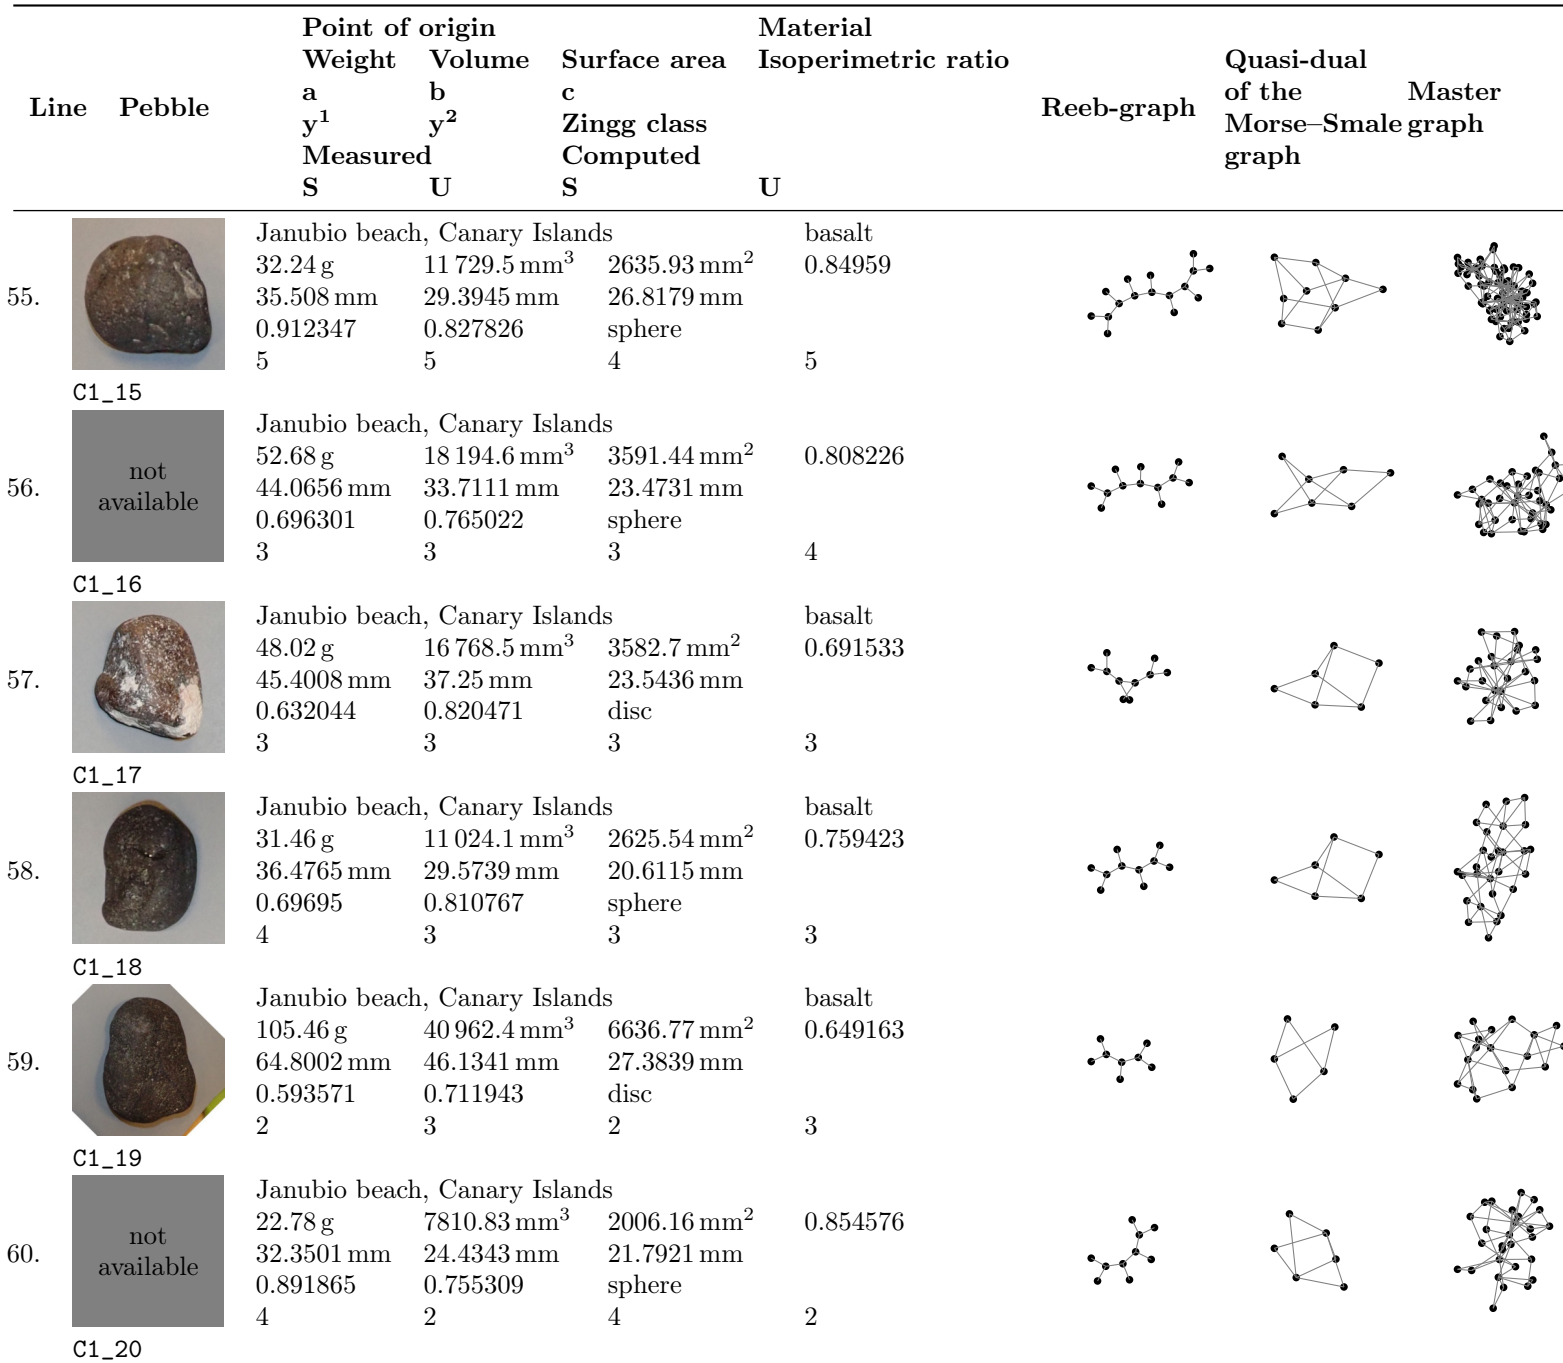 | 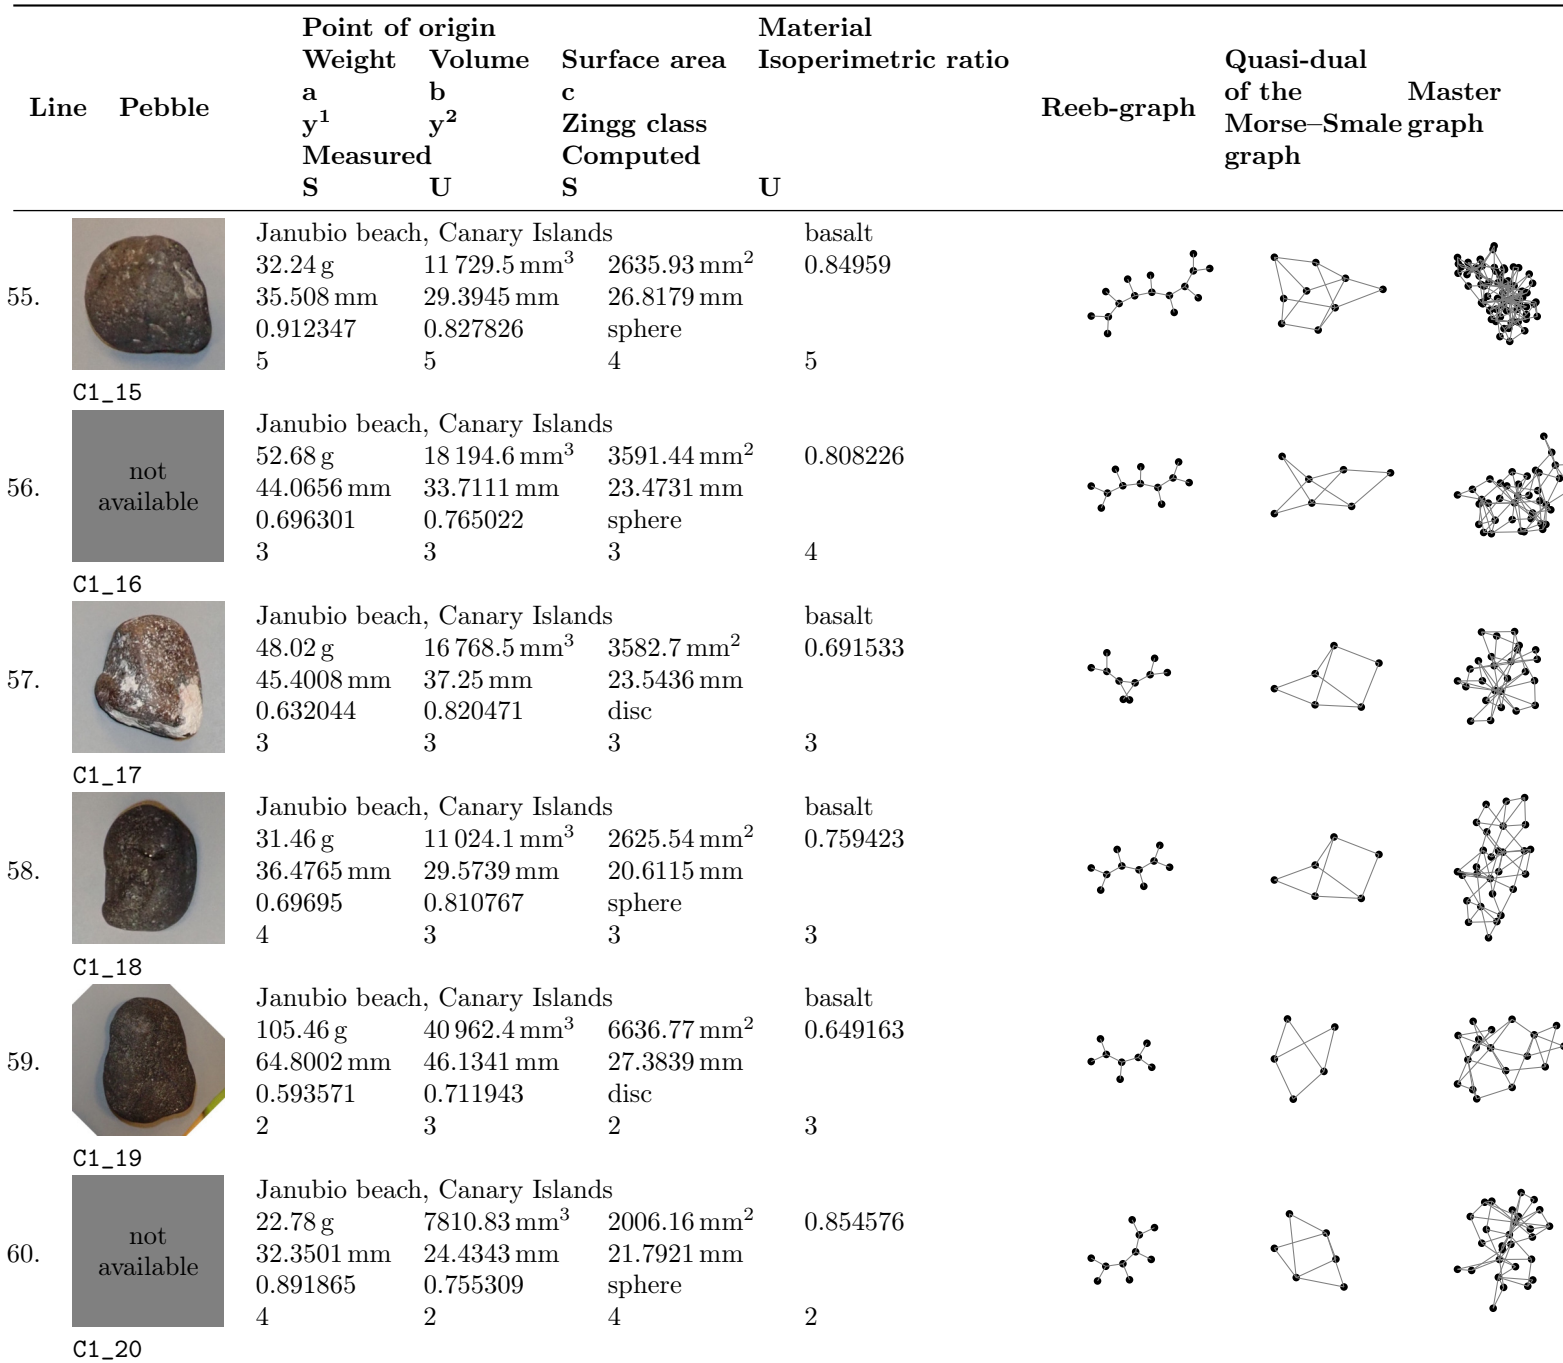 | 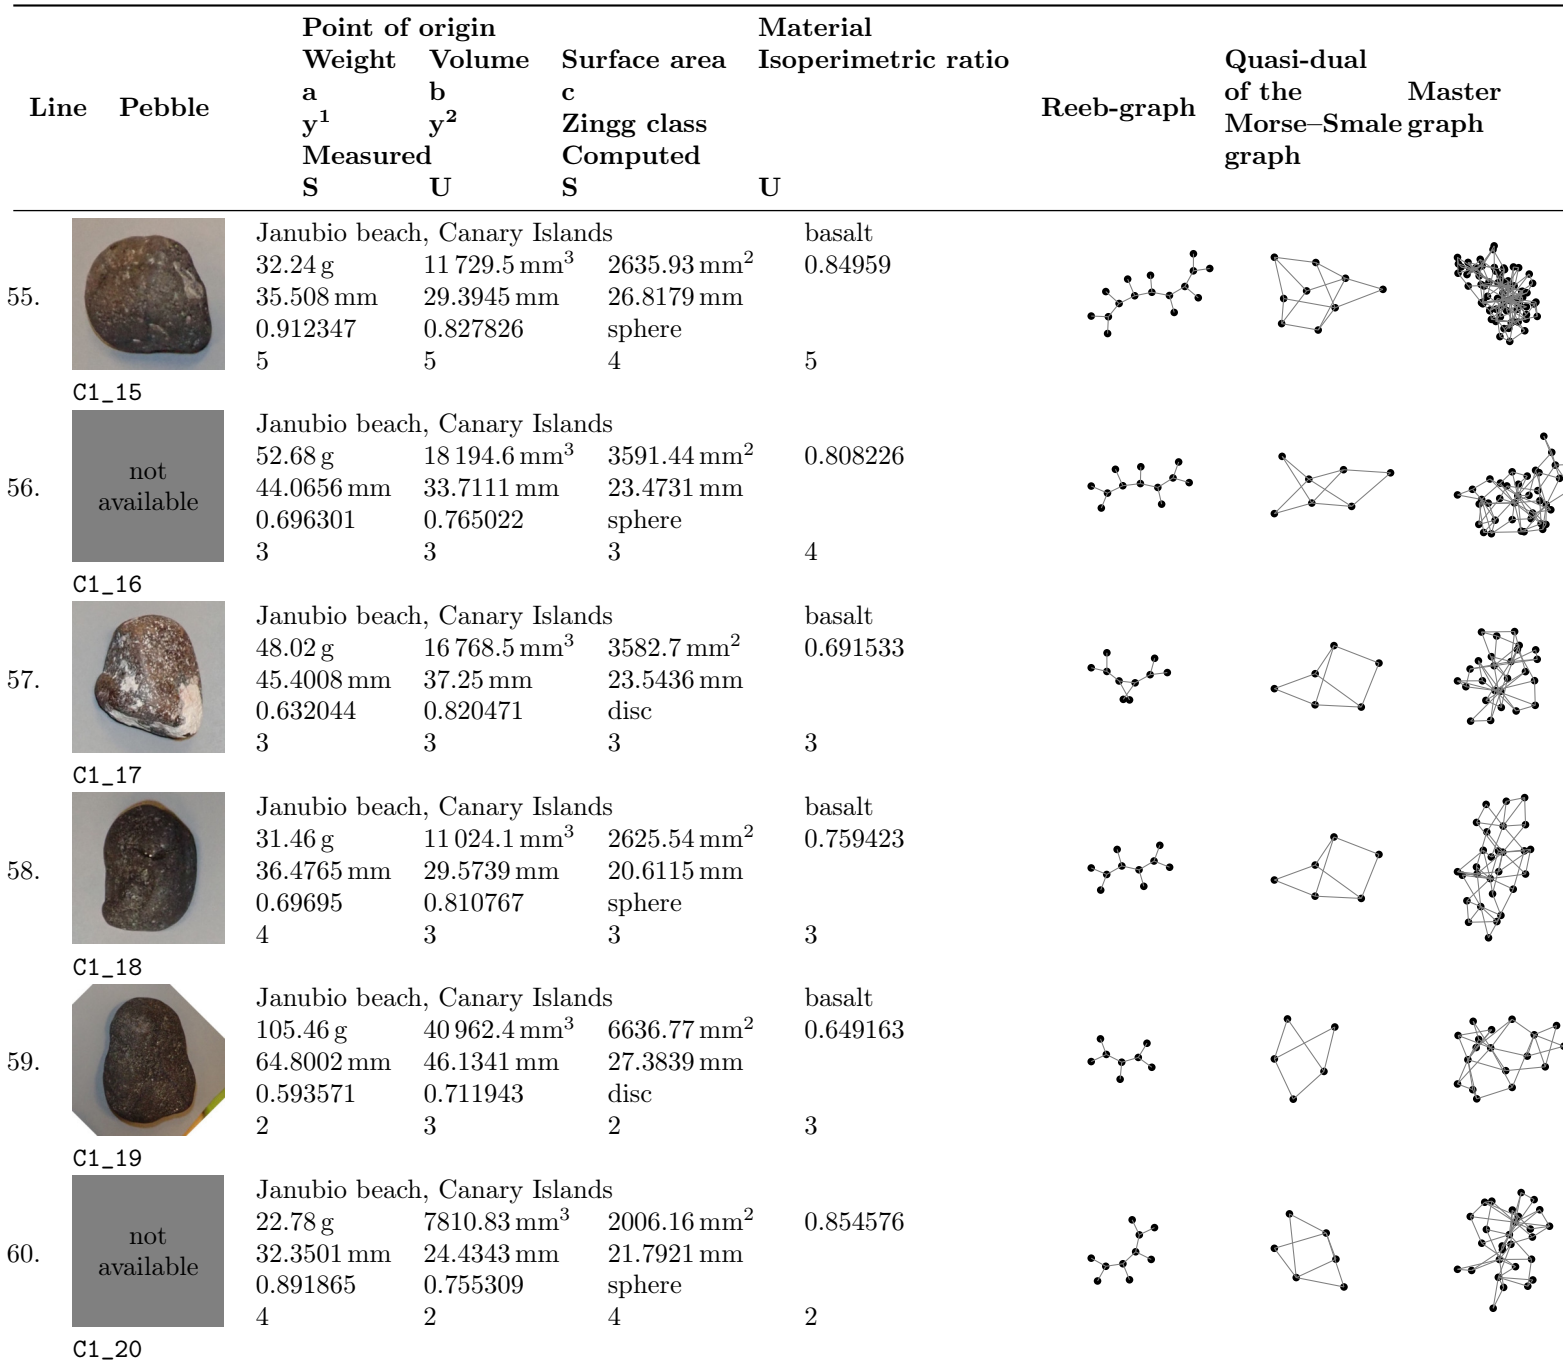 |                 |
|       | 22.78 g                                                                             | 7810.83 mm <sup>3</sup>              | 2006.16 mm <sup>2</sup>  | 0.854576                          |          |                                                                                       |                                                                                       |                                                                                       |                 |
|       | 32.3501 mm                                                                          | 24.4343 mm                           | 21.7921 mm               |                                   |          |                                                                                       |                                                                                       |                                                                                       |                 |
|       | 0.891865                                                                            | 0.755309                             | sphere                   |                                   |          |                                                                                       |                                                                                       |                                                                                       |                 |
|       | 4                                                                                   | 2                                    | 4                        | 2                                 |          |                                                                                       |                                                                                       |                                                                                       |                 |
| C1_20 |                                                                                     |                                      |                          |                                   |          |                                                                                       |                                                                                       |                                                                                       |                 |

| Line  | Pebble                                                                              | Point of origin               |                          |                         | Material | Isoperimetric ratio                                                                   | Reeb-graph                                                                            | Quasi-dual<br>of the<br>Morse–Smale<br>graph                                          | Master<br>graph |
|-------|-------------------------------------------------------------------------------------|-------------------------------|--------------------------|-------------------------|----------|---------------------------------------------------------------------------------------|---------------------------------------------------------------------------------------|---------------------------------------------------------------------------------------|-----------------|
|       |                                                                                     | Weight                        | Volume                   | Surface area            |          |                                                                                       |                                                                                       |                                                                                       |                 |
|       |                                                                                     | a                             | b                        | c                       |          |                                                                                       |                                                                                       |                                                                                       |                 |
|       |                                                                                     | y <sup>1</sup>                | y <sup>2</sup>           | Zingg class             |          |                                                                                       |                                                                                       |                                                                                       |                 |
|       |                                                                                     | Measured                      | U                        | Computed                | U        |                                                                                       |                                                                                       |                                                                                       |                 |
|       |                                                                                     | S                             | U                        | S                       | U        |                                                                                       |                                                                                       |                                                                                       |                 |
| 61.   | 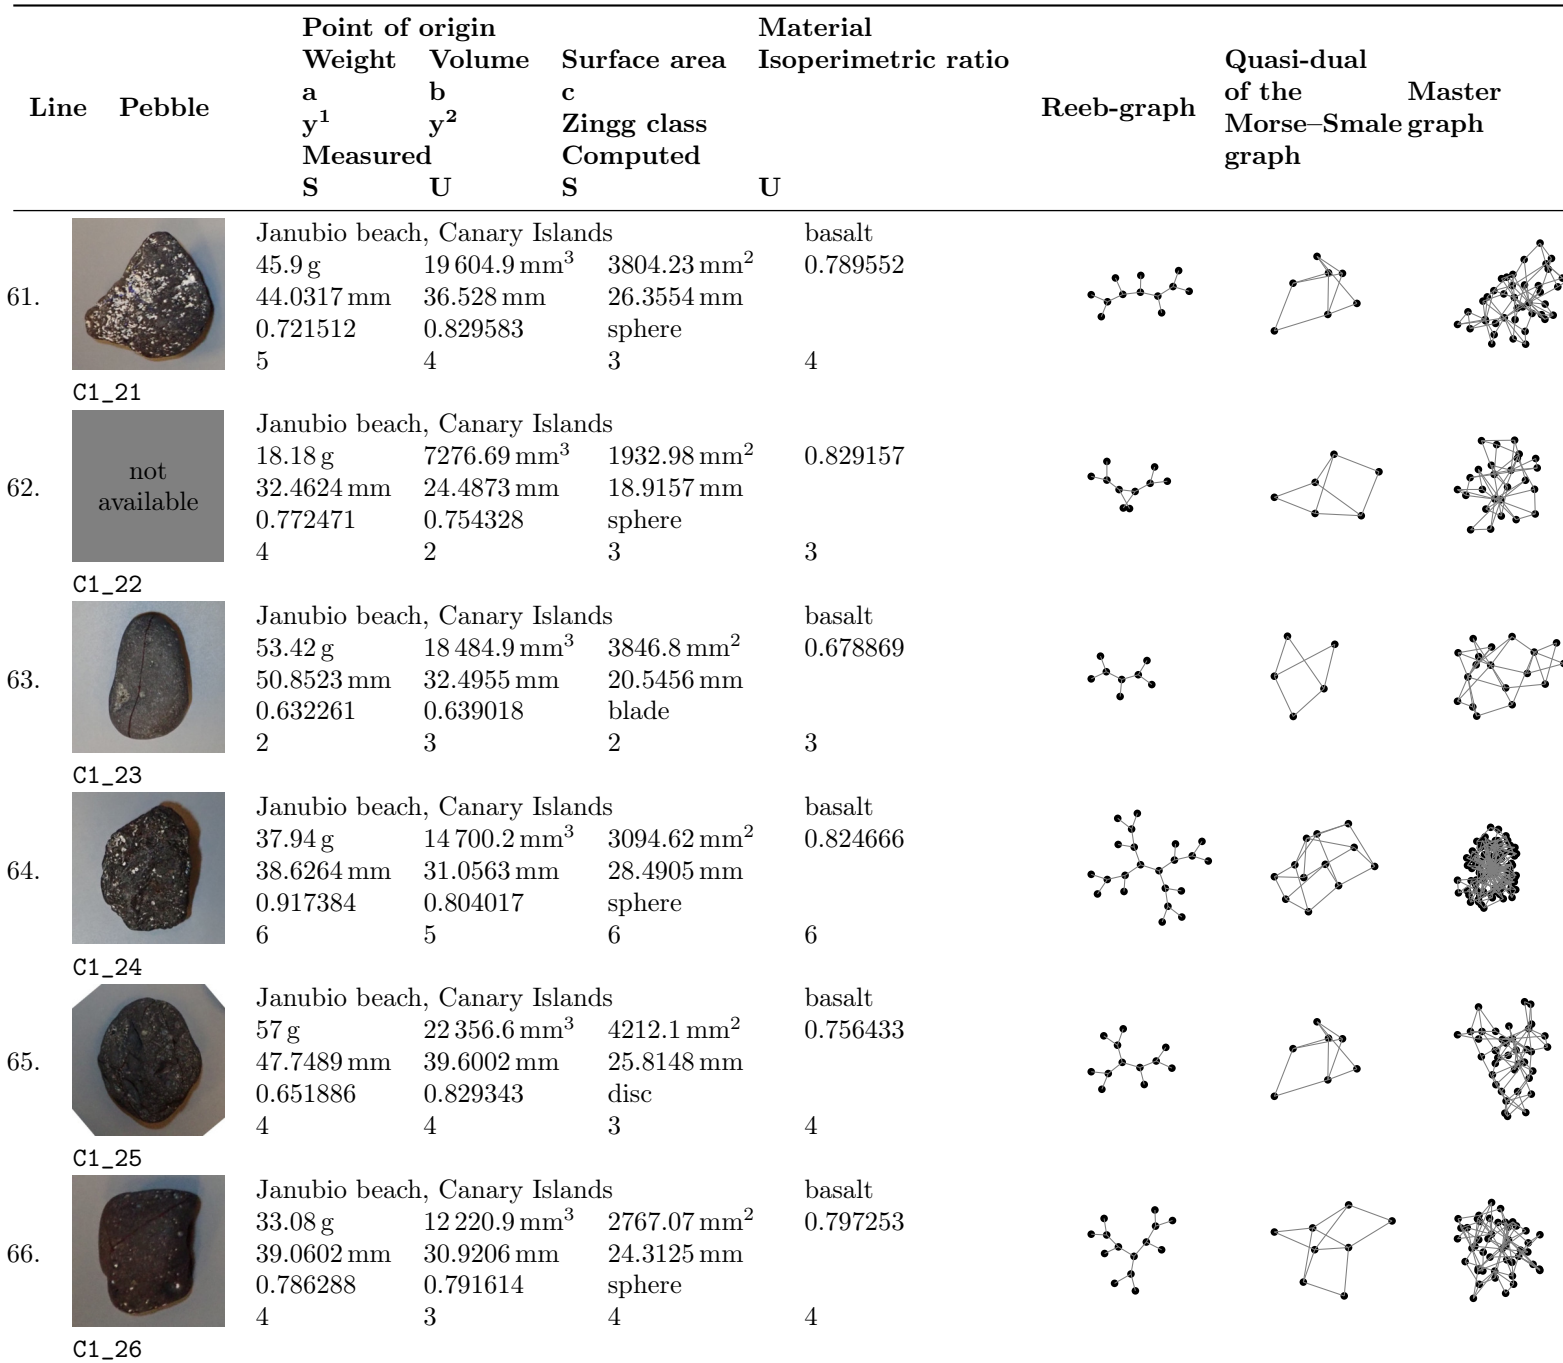   | Janubio beach, Canary Islands |                          |                         | basalt   | 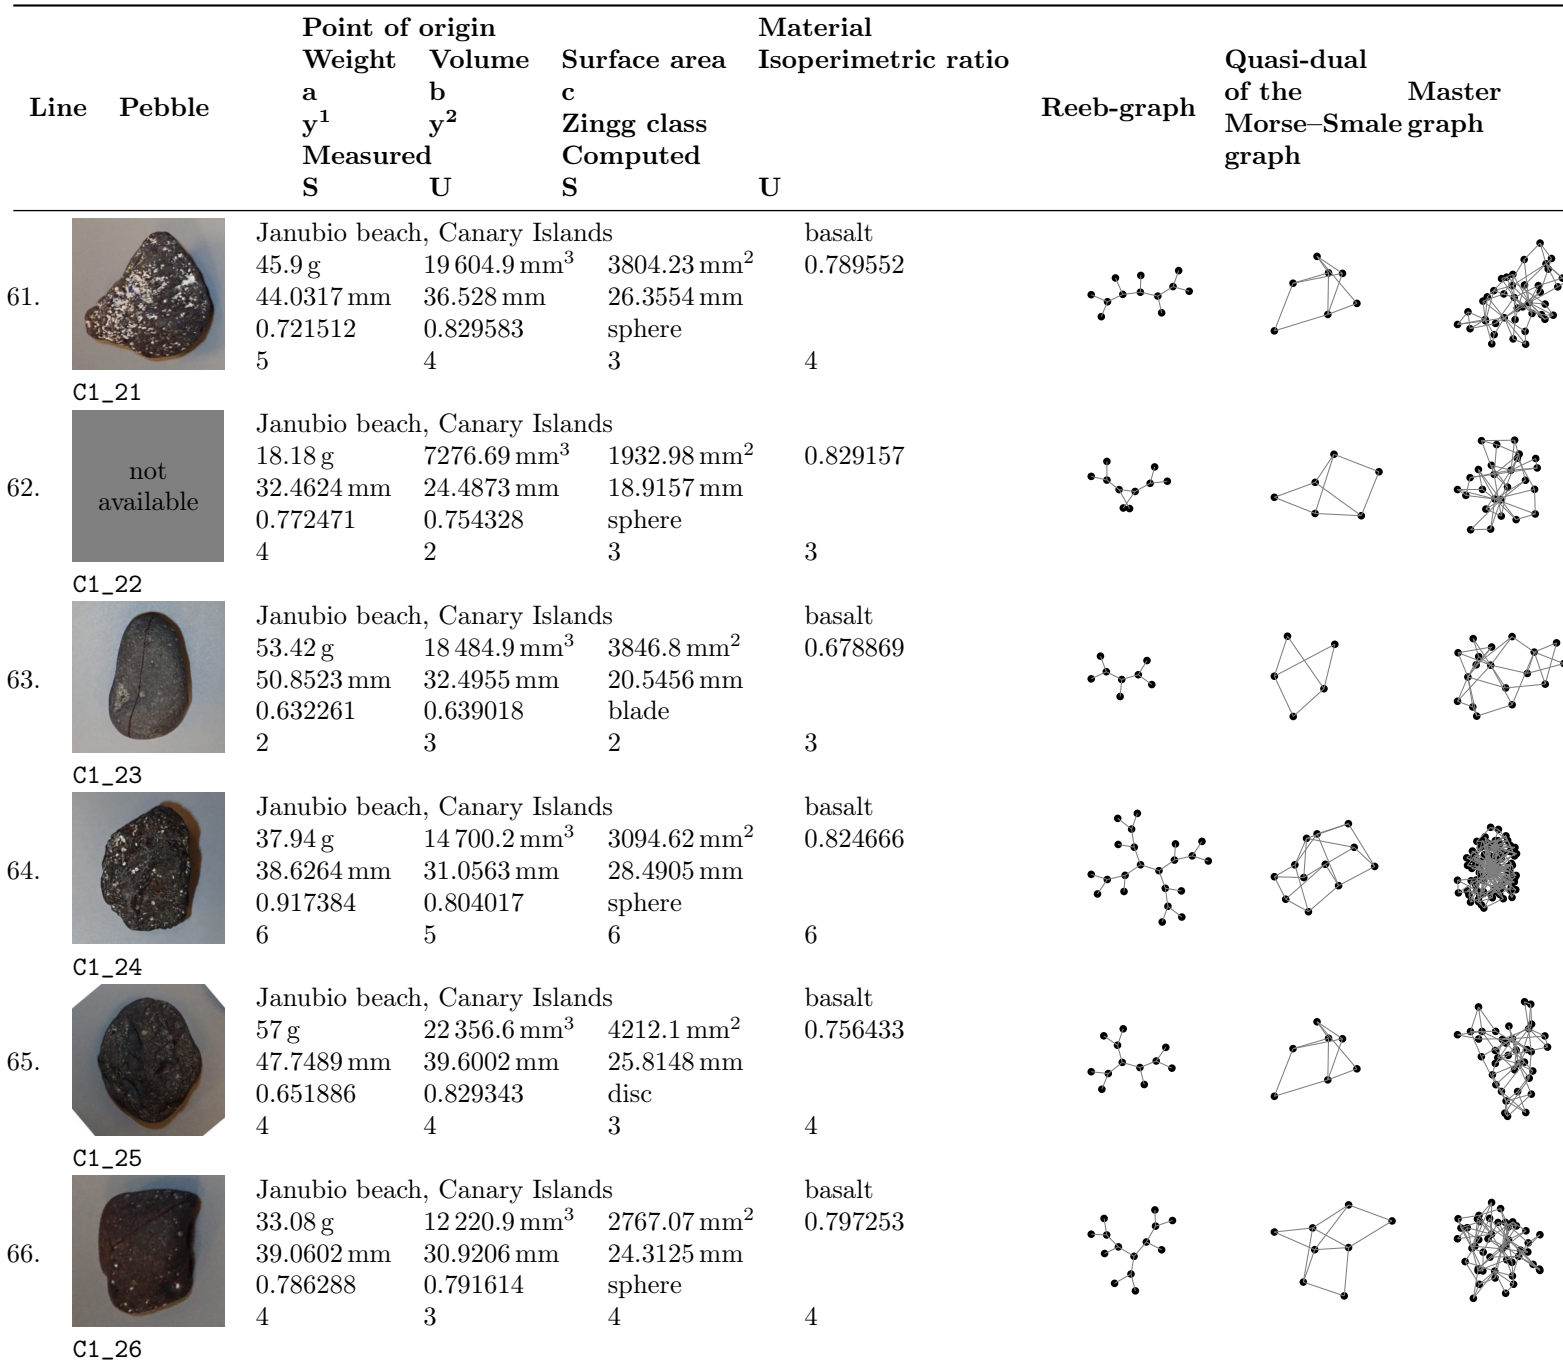   | 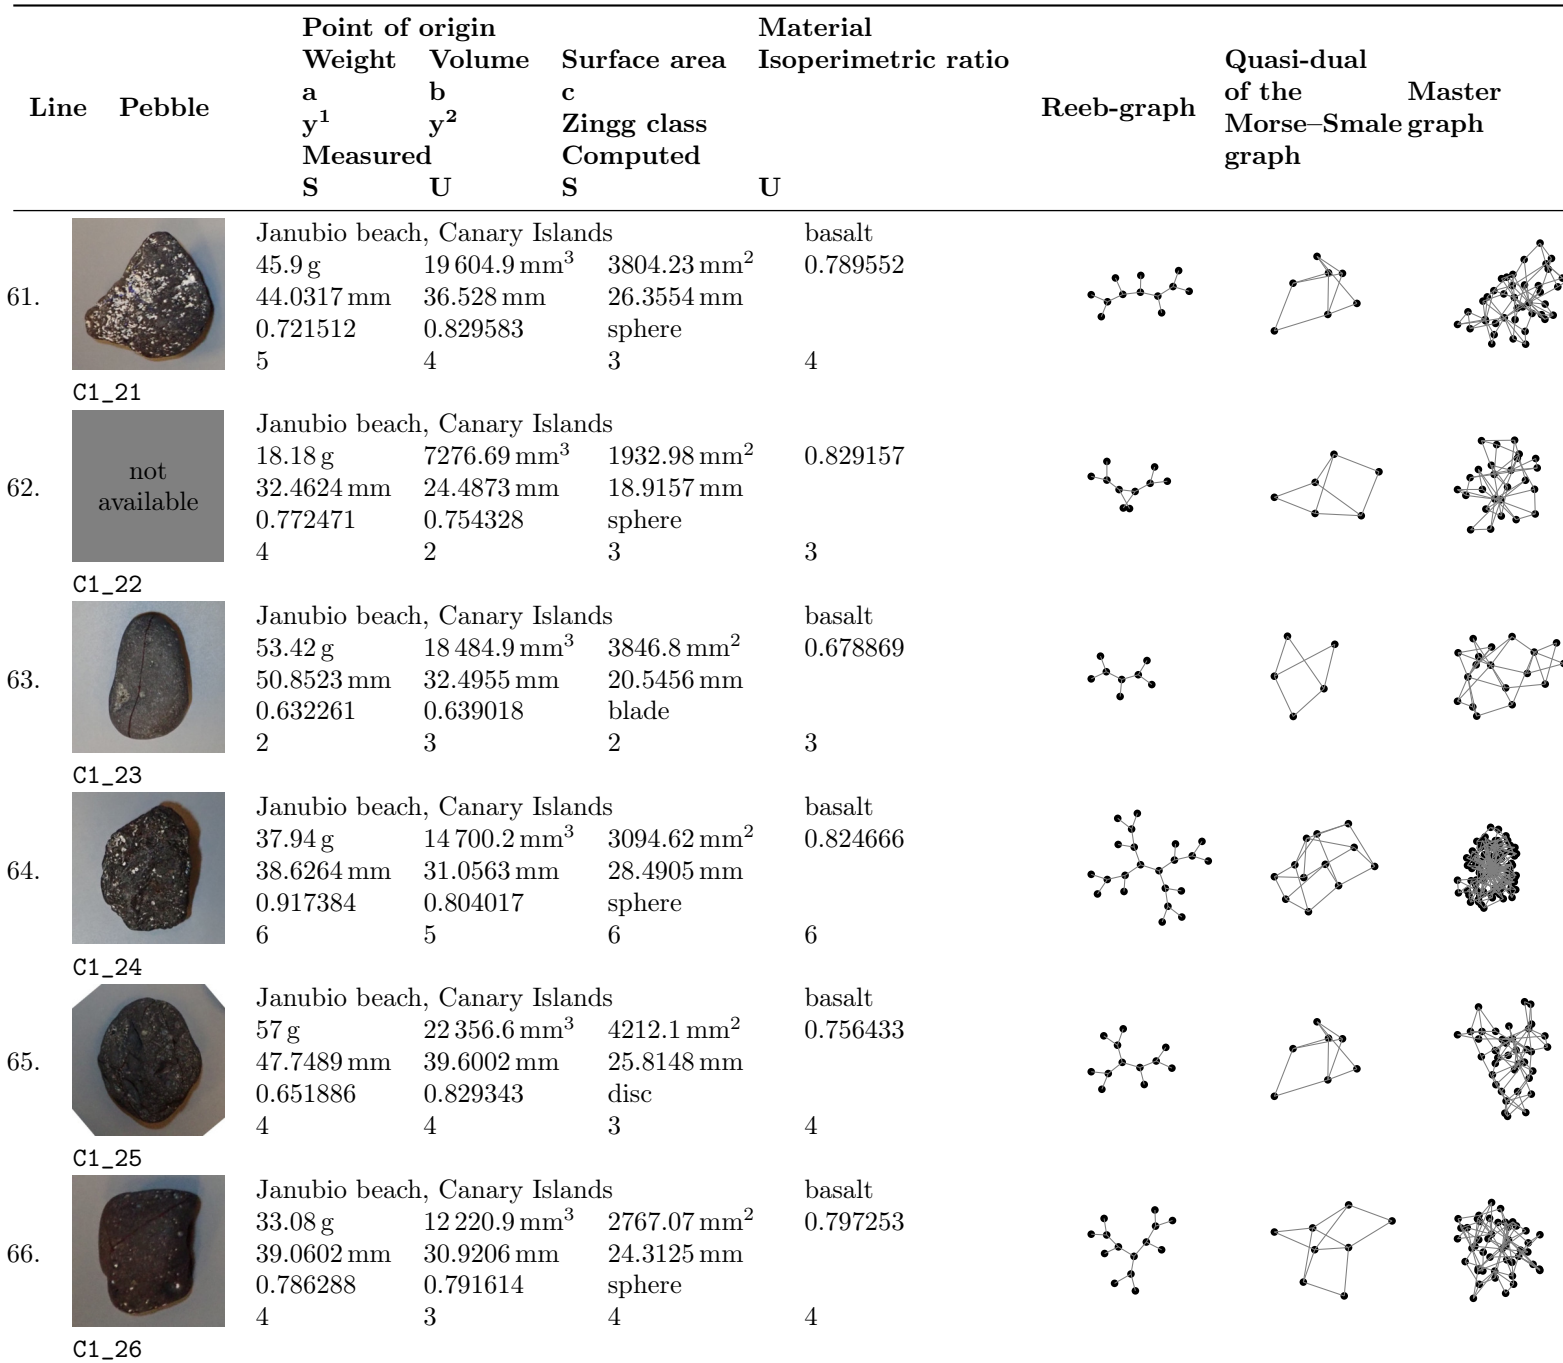   | 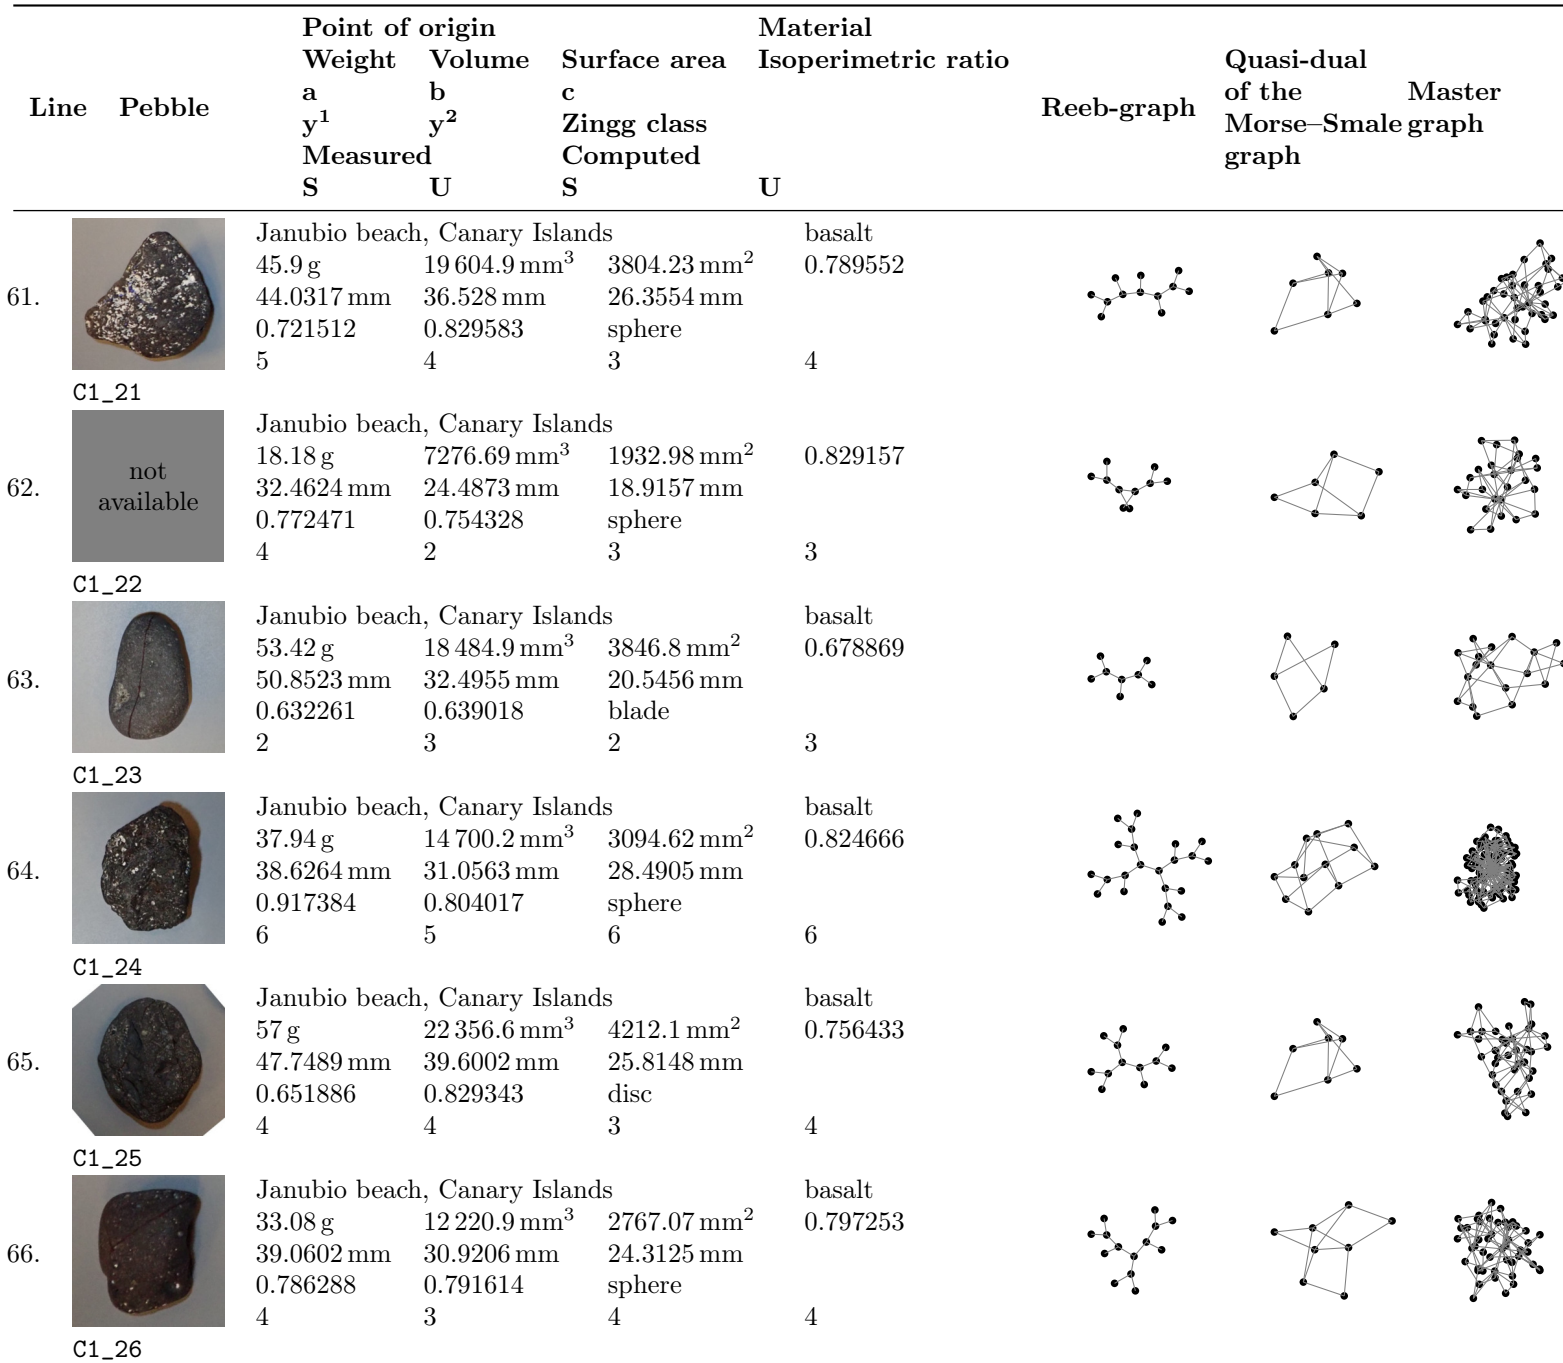   |                 |
|       |                                                                                     | 45.9 g                        | 19 604.9 mm <sup>3</sup> | 3804.23 mm <sup>2</sup> | 0.789552 |                                                                                       |                                                                                       |                                                                                       |                 |
|       |                                                                                     | 44.0317 mm                    | 36.528 mm                | 26.3554 mm              |          |                                                                                       |                                                                                       |                                                                                       |                 |
|       |                                                                                     | 0.721512                      | 0.829583                 | sphere                  |          |                                                                                       |                                                                                       |                                                                                       |                 |
|       |                                                                                     | 5                             | 4                        | 3                       | 4        |                                                                                       |                                                                                       |                                                                                       |                 |
| C1_21 |                                                                                     |                               |                          |                         |          |                                                                                       |                                                                                       |                                                                                       |                 |
| 62.   | 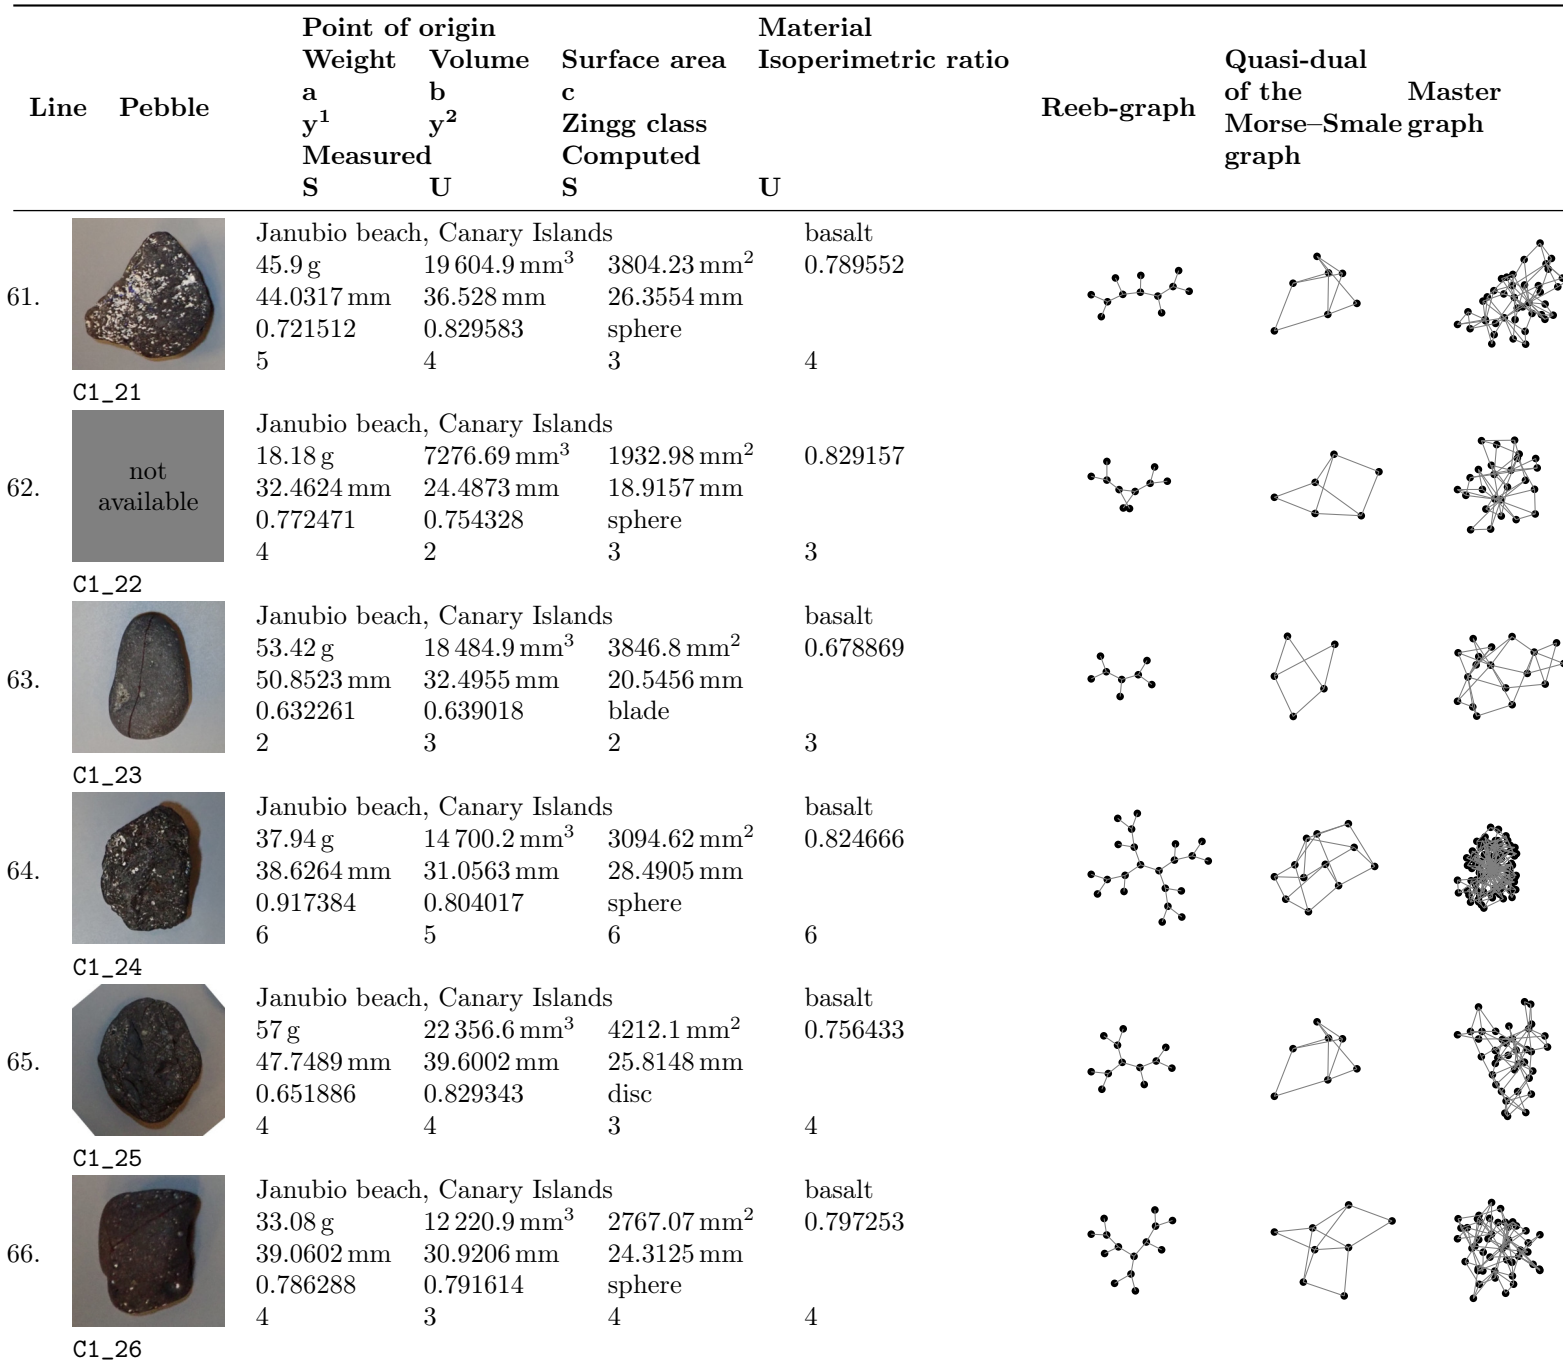   | Janubio beach, Canary Islands |                          |                         |          | 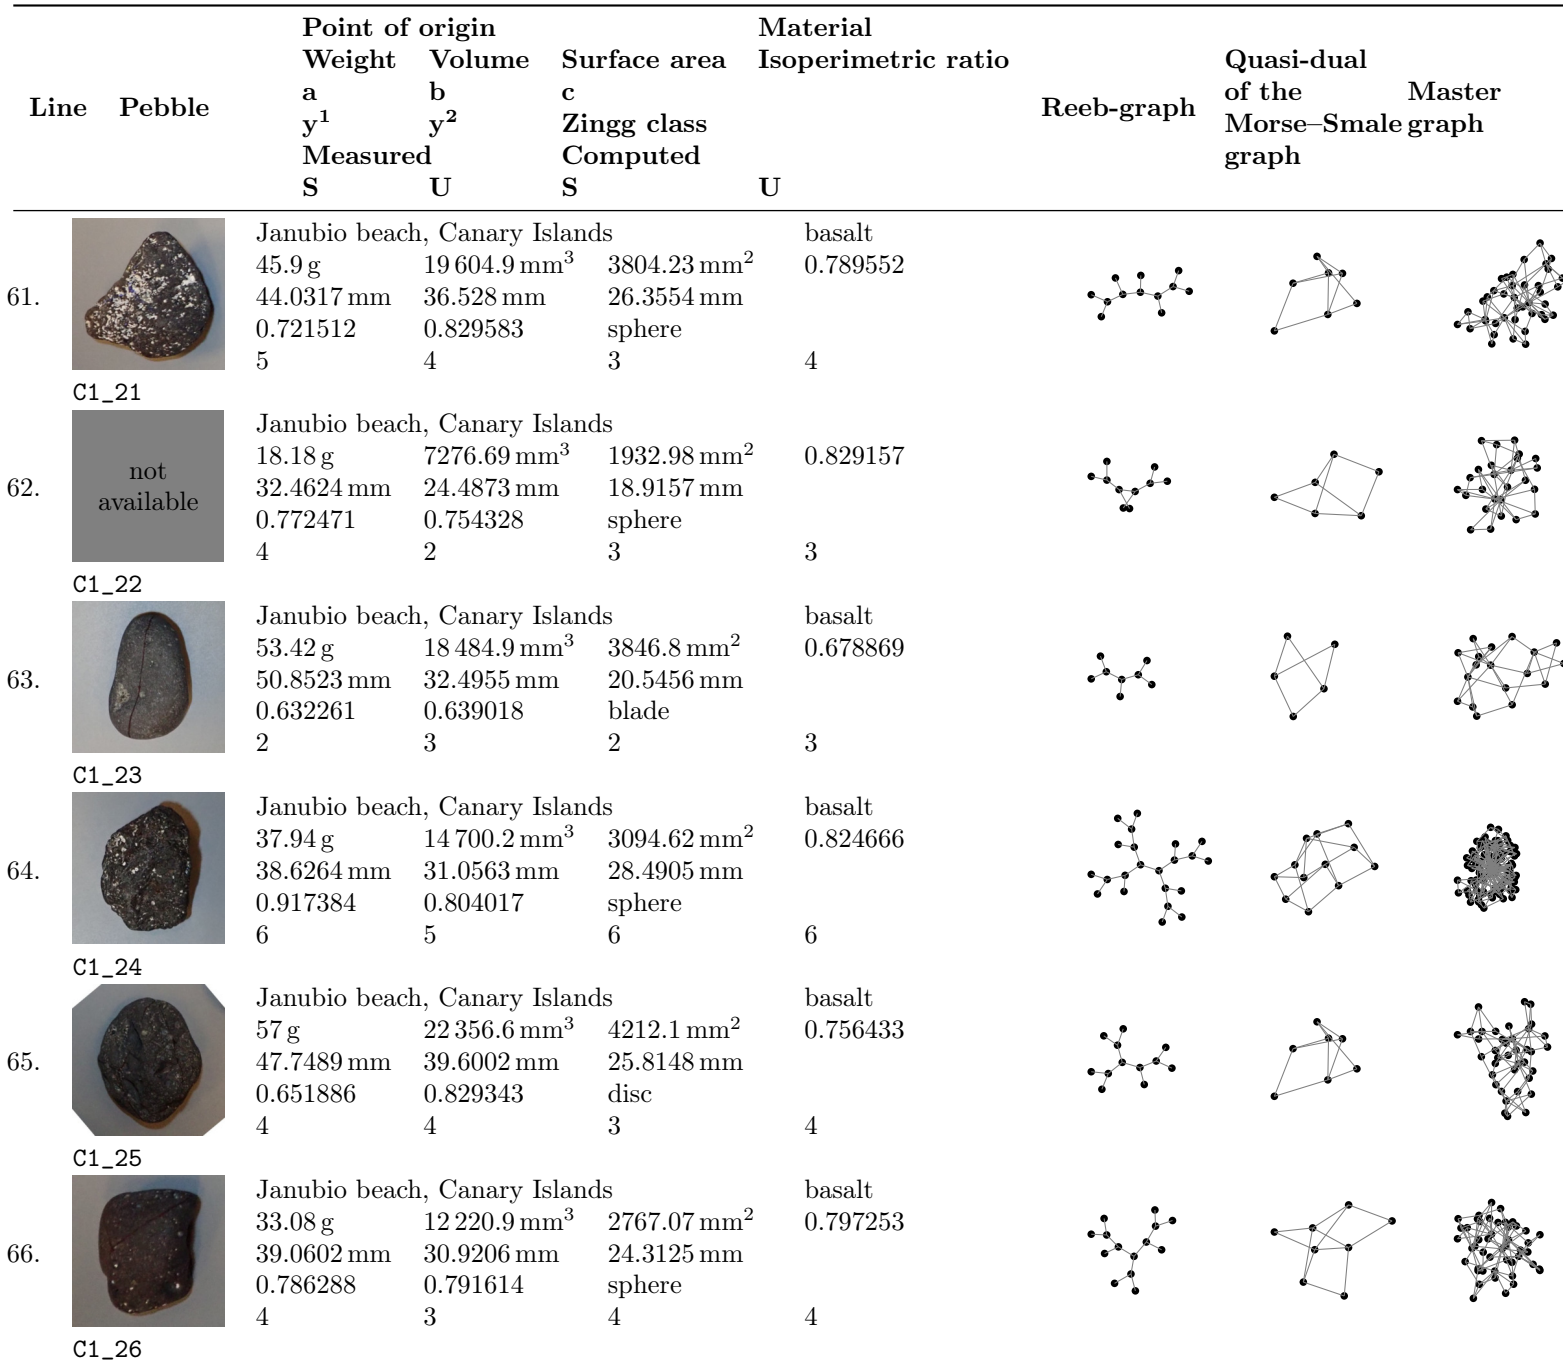   | 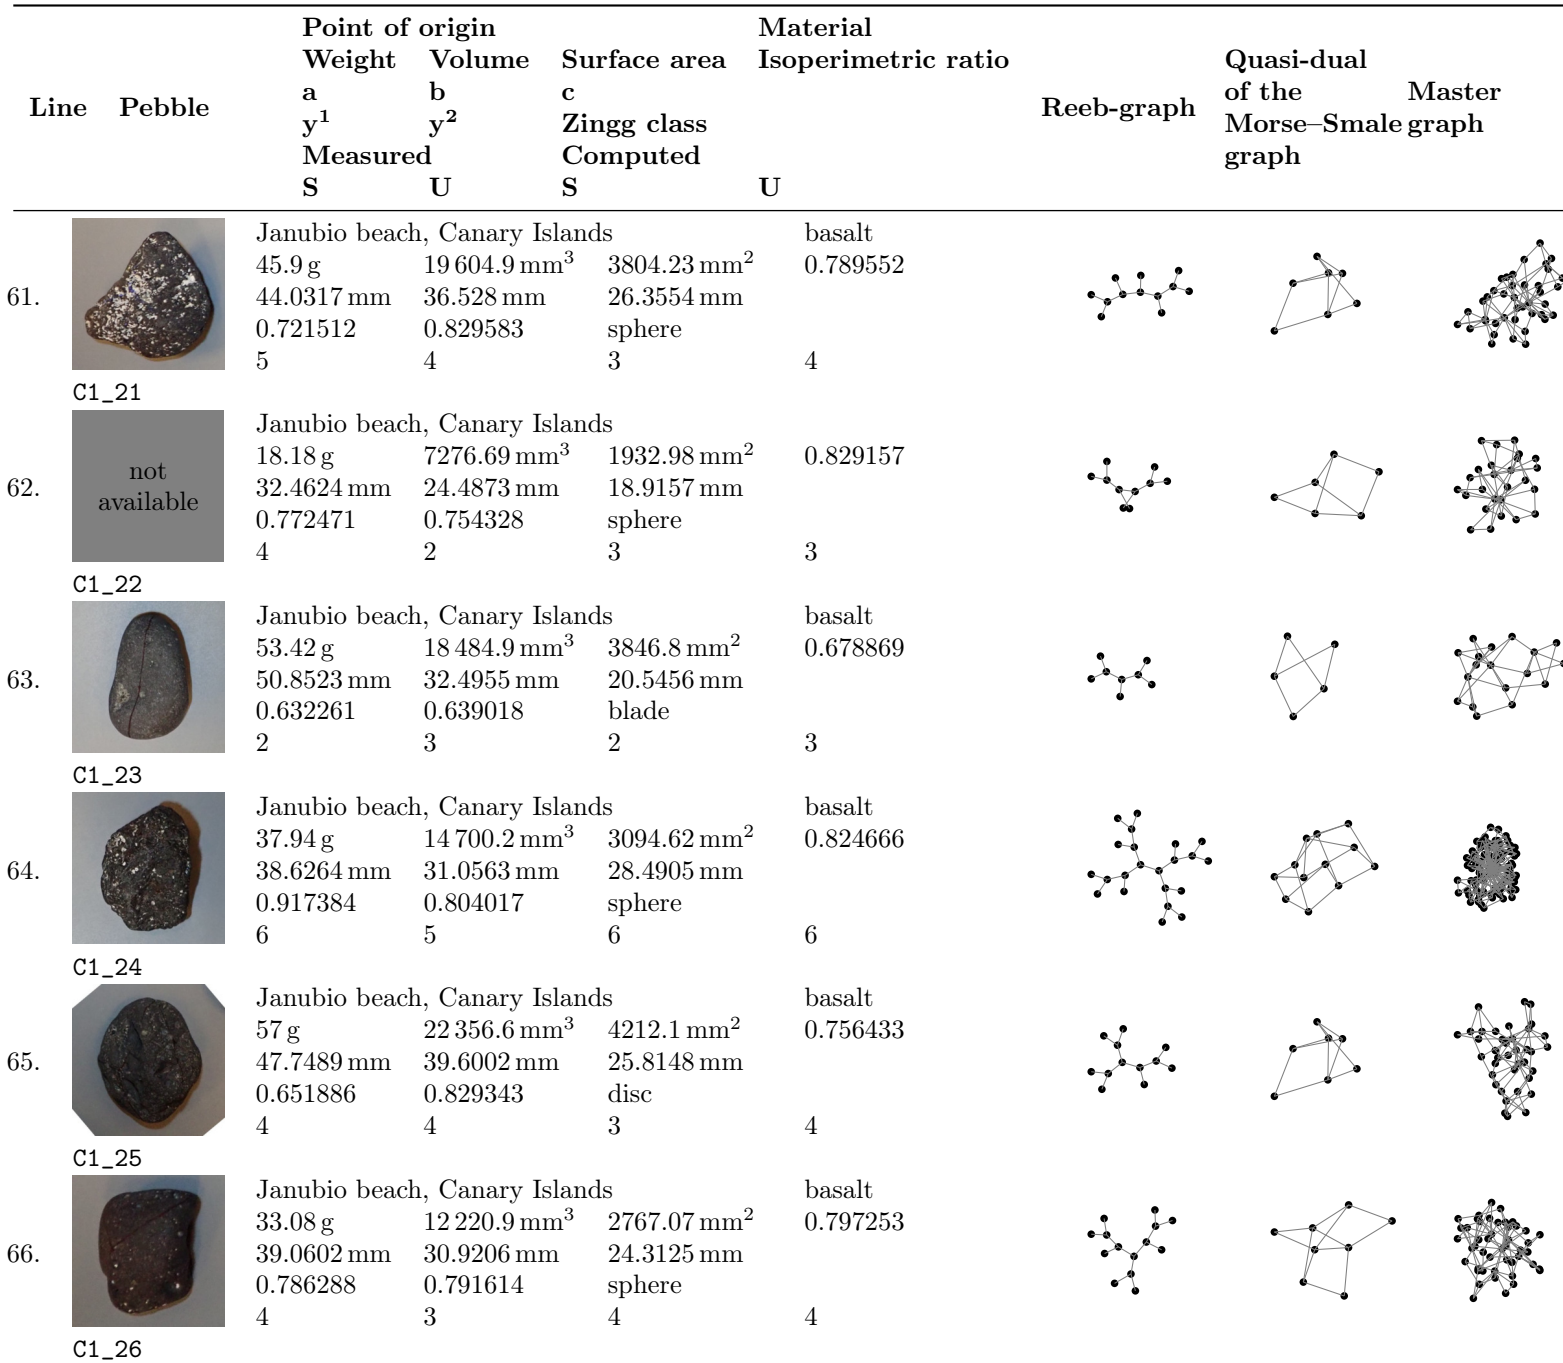   | 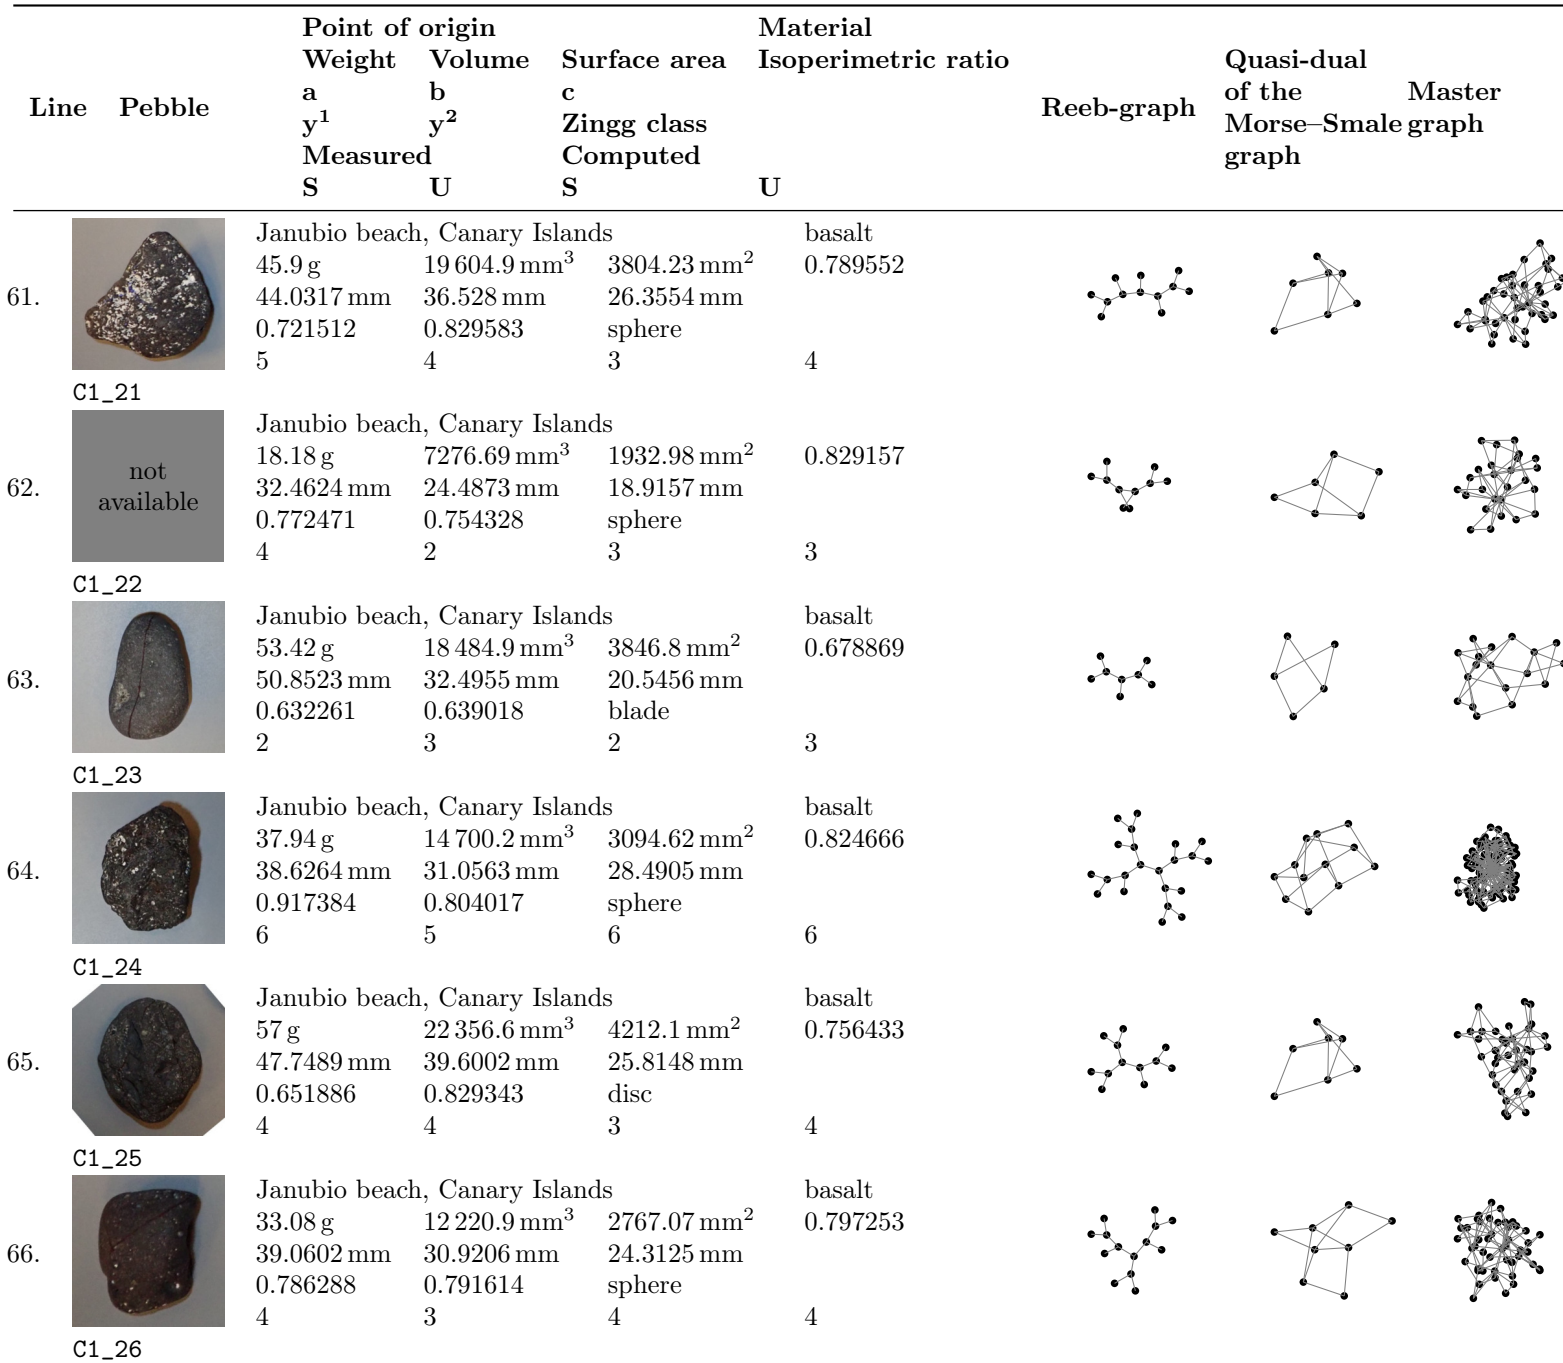   |                 |
|       |                                                                                     | 18.18 g                       | 7276.69 mm <sup>3</sup>  | 1932.98 mm <sup>2</sup> | 0.829157 |                                                                                       |                                                                                       |                                                                                       |                 |
|       |                                                                                     | 32.4624 mm                    | 24.4873 mm               | 18.9157 mm              |          |                                                                                       |                                                                                       |                                                                                       |                 |
|       |                                                                                     | 0.772471                      | 0.754328                 | sphere                  |          |                                                                                       |                                                                                       |                                                                                       |                 |
|       |                                                                                     | 4                             | 2                        | 3                       | 3        |                                                                                       |                                                                                       |                                                                                       |                 |
| C1_22 |                                                                                     |                               |                          |                         |          |                                                                                       |                                                                                       |                                                                                       |                 |
| 63.   | 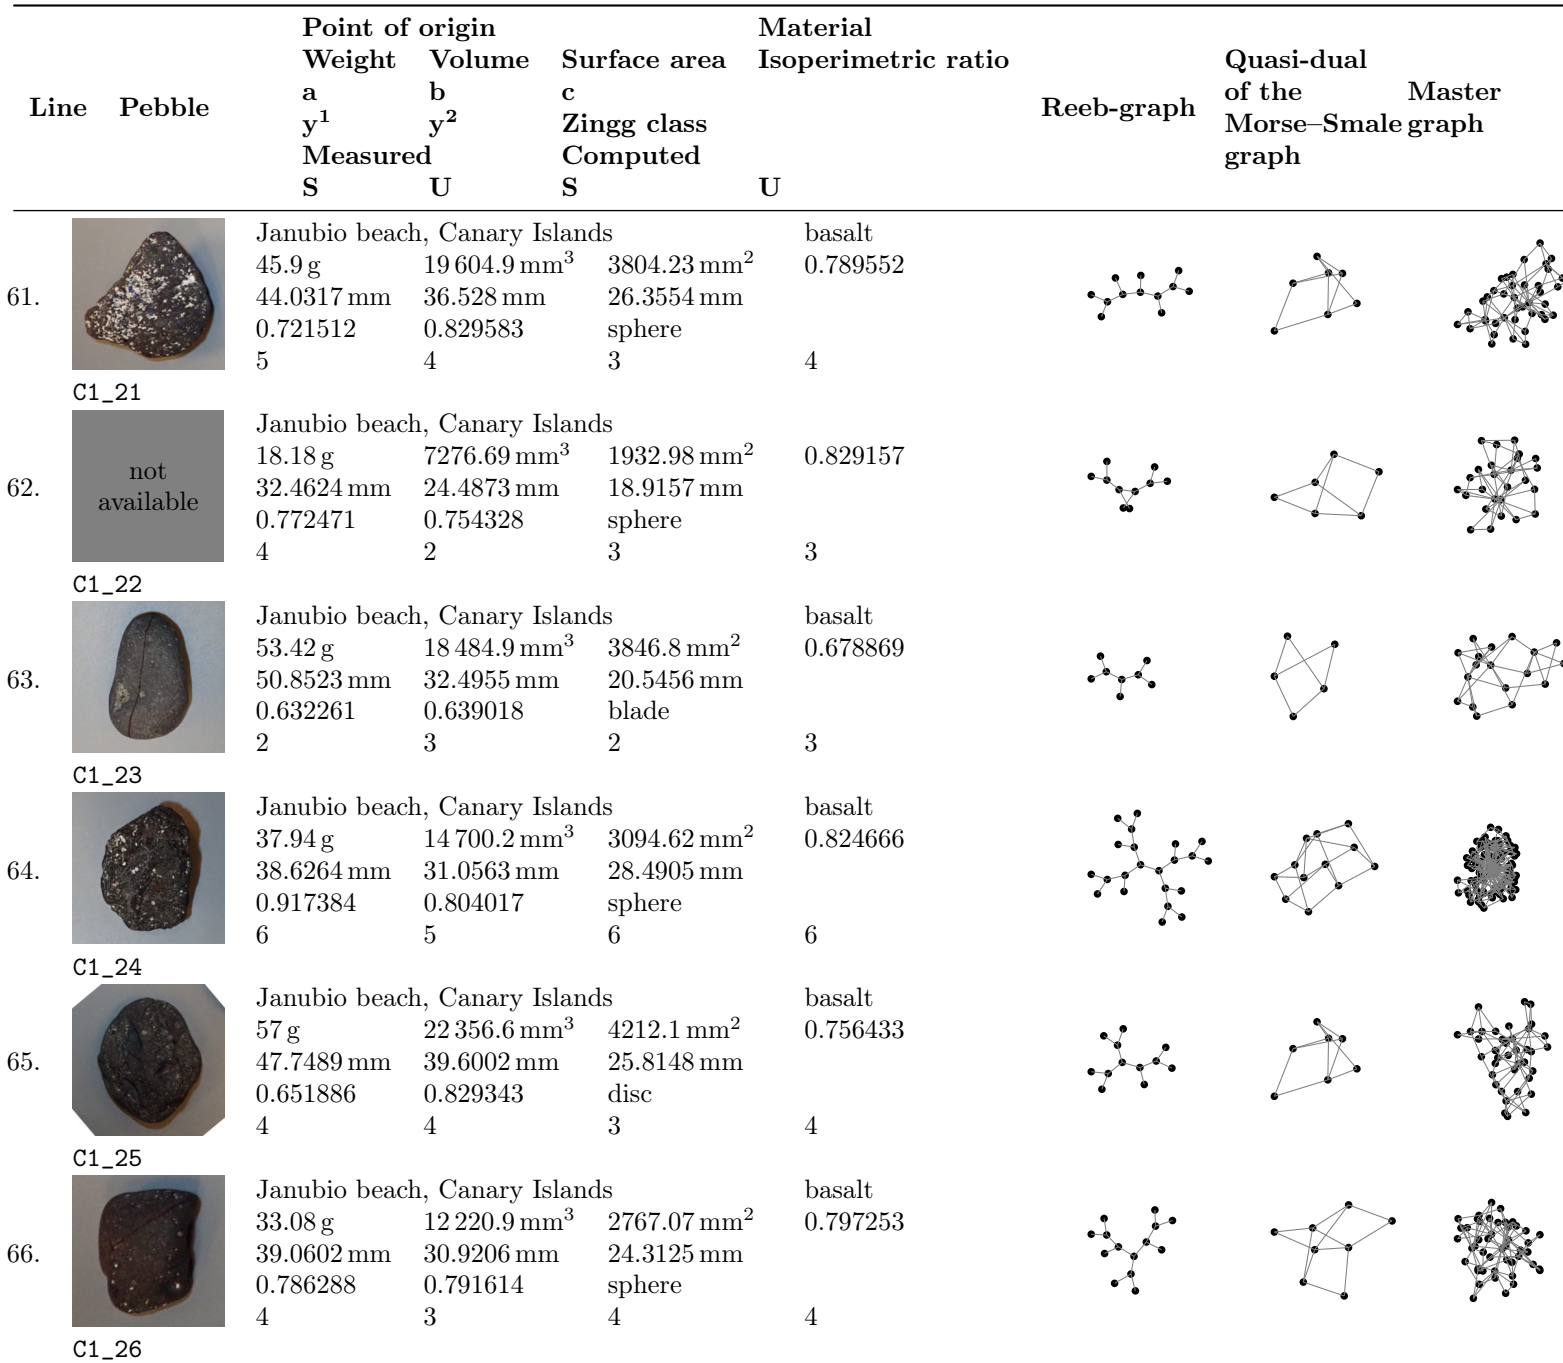   | Janubio beach, Canary Islands |                          |                         | basalt   | 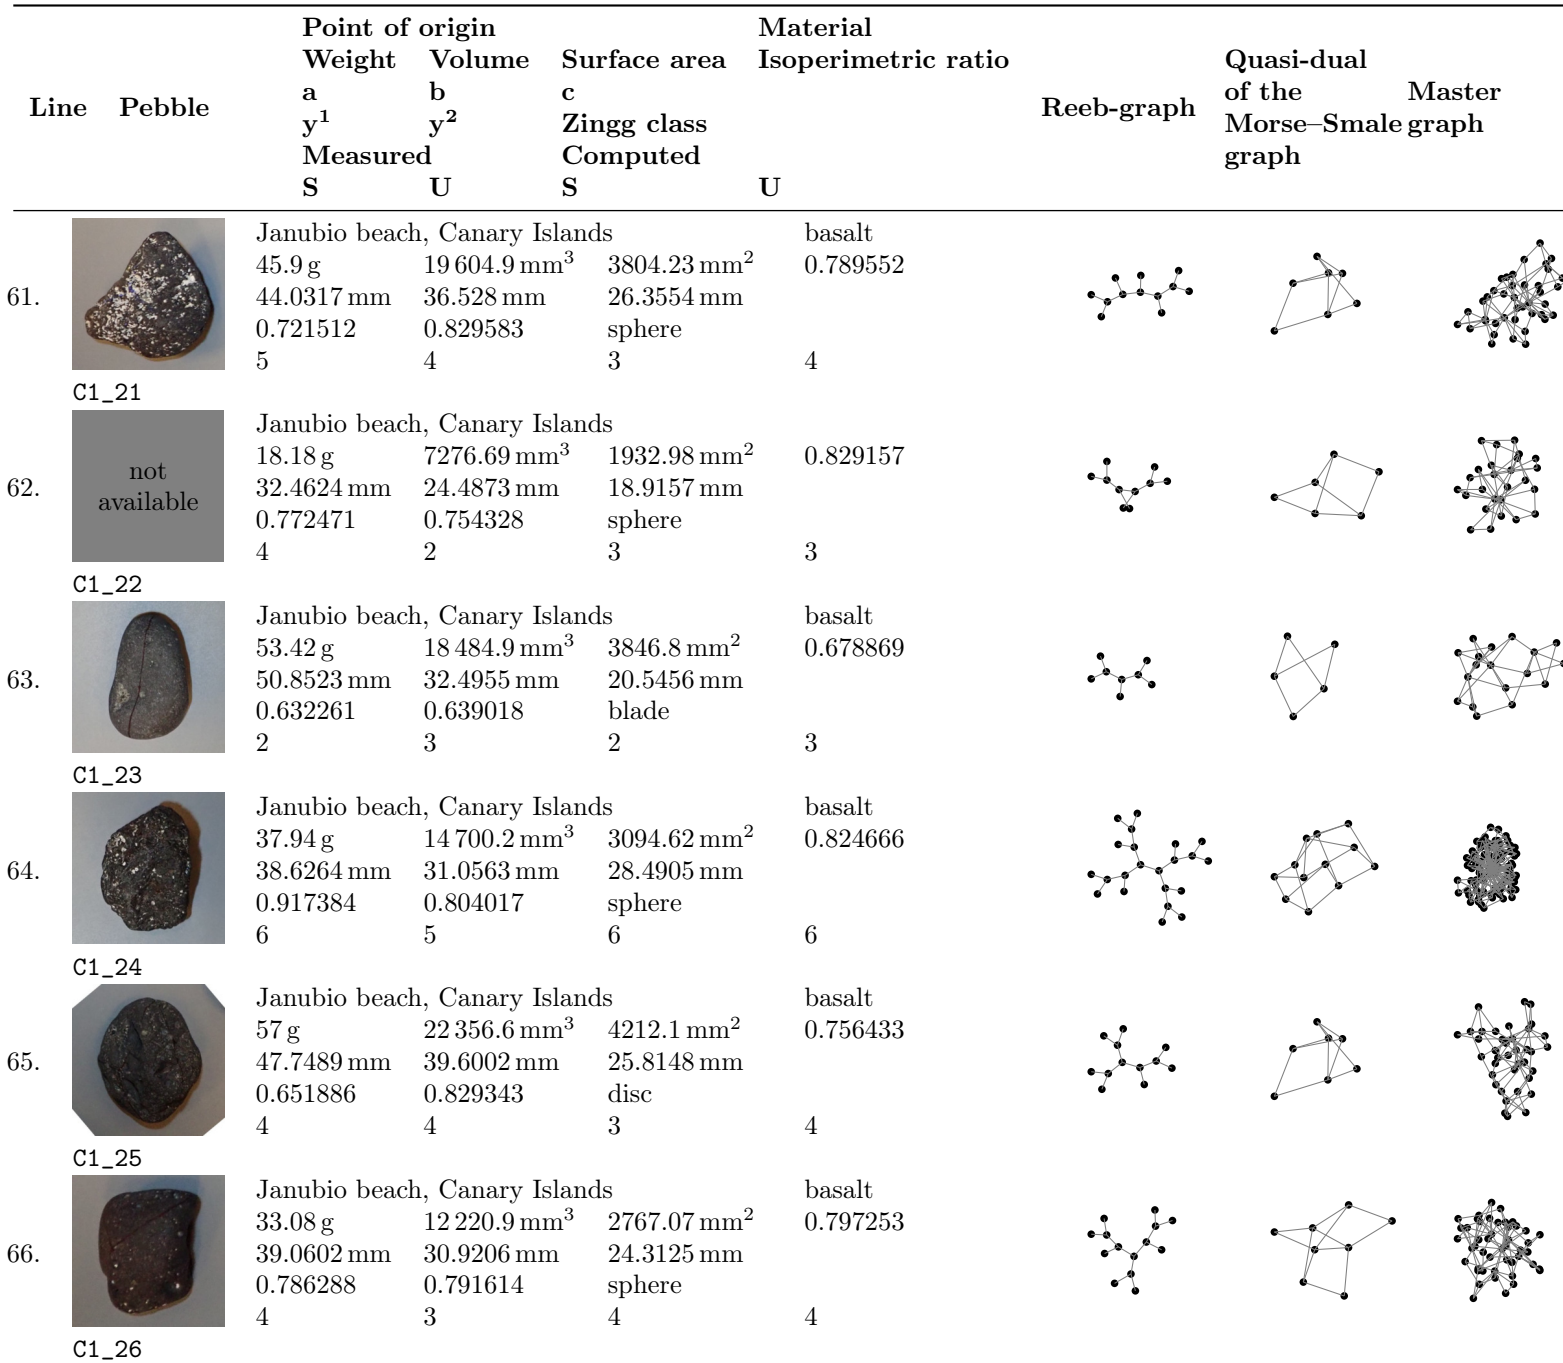   | 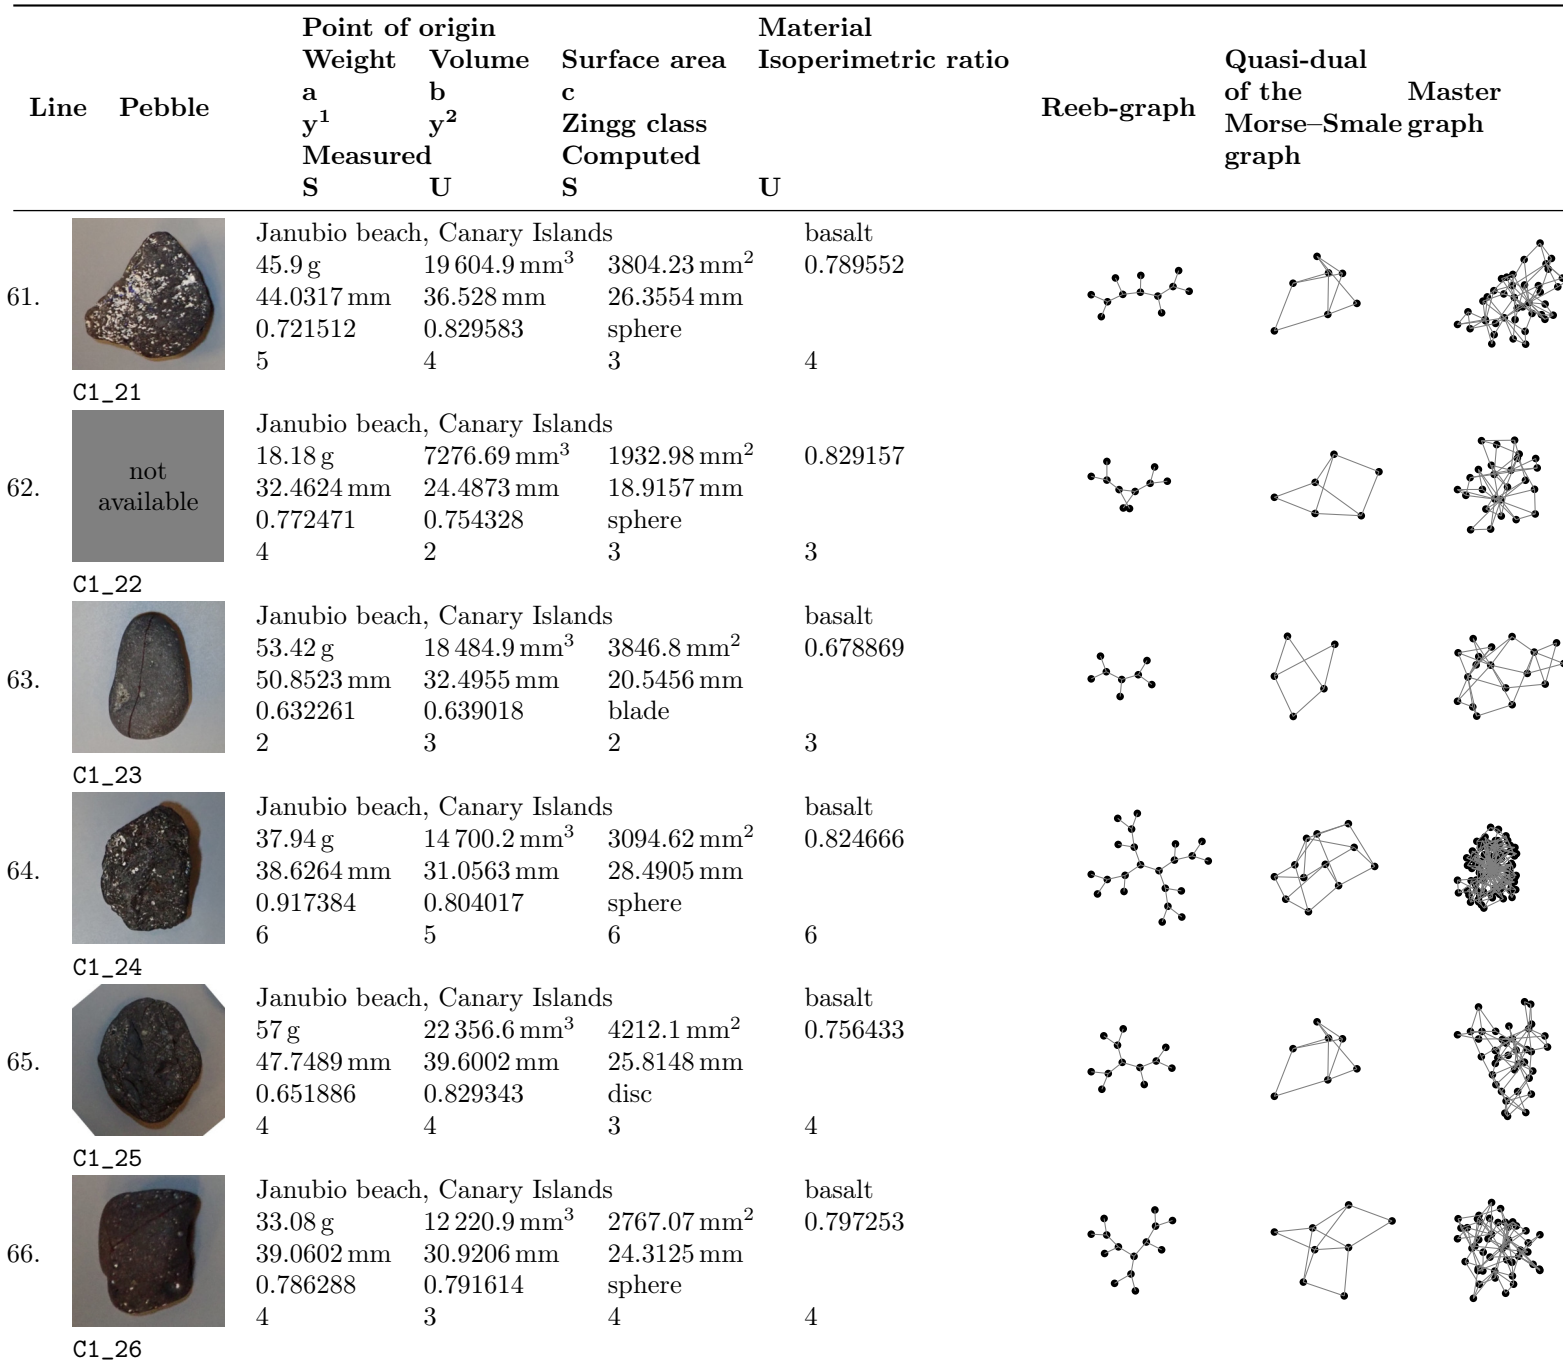   | 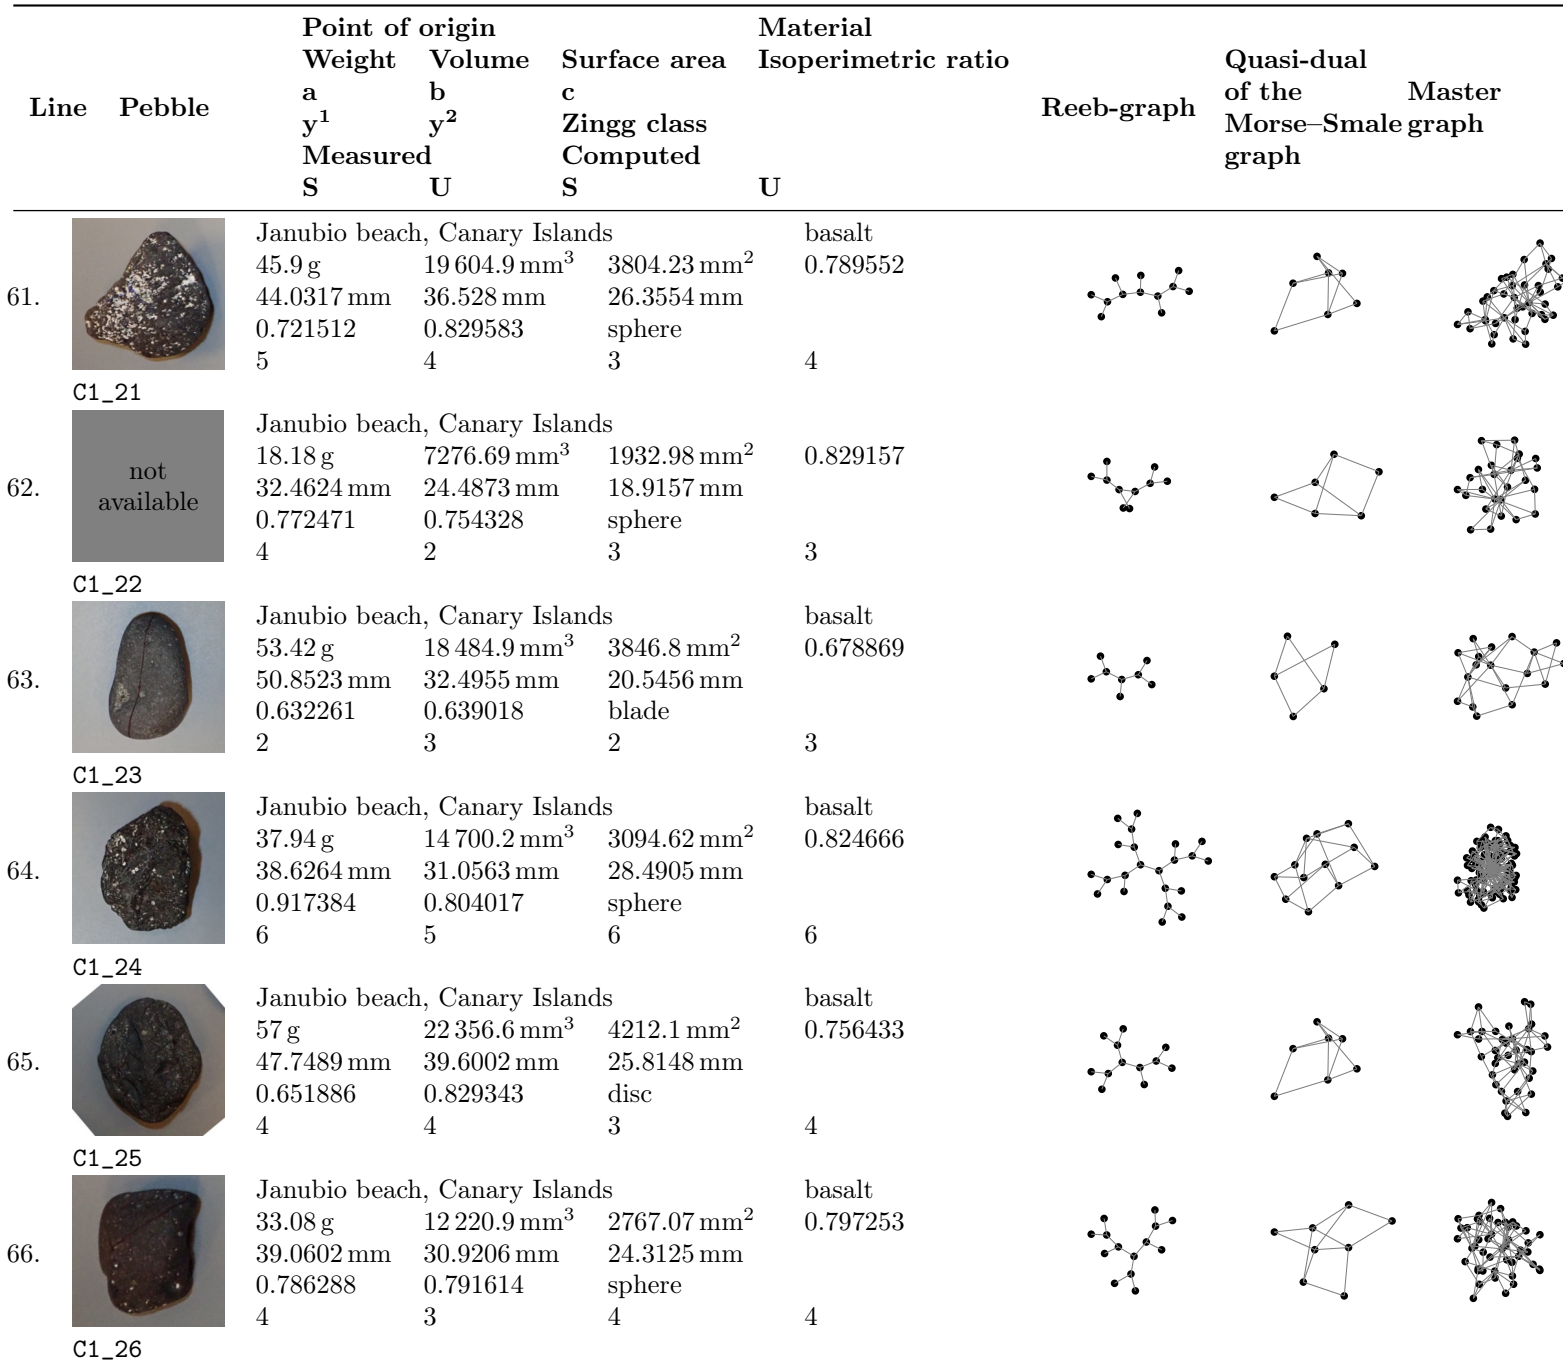   |                 |
|       |                                                                                     | 53.42 g                       | 18 484.9 mm <sup>3</sup> | 3846.8 mm <sup>2</sup>  | 0.678869 |                                                                                       |                                                                                       |                                                                                       |                 |
|       |                                                                                     | 50.8523 mm                    | 32.4955 mm               | 20.5456 mm              |          |                                                                                       |                                                                                       |                                                                                       |                 |
|       |                                                                                     | 0.632261                      | 0.639018                 | blade                   |          |                                                                                       |                                                                                       |                                                                                       |                 |
|       |                                                                                     | 2                             | 3                        | 2                       | 3        |                                                                                       |                                                                                       |                                                                                       |                 |
| C1_23 |                                                                                     |                               |                          |                         |          |                                                                                       |                                                                                       |                                                                                       |                 |
| 64.   | 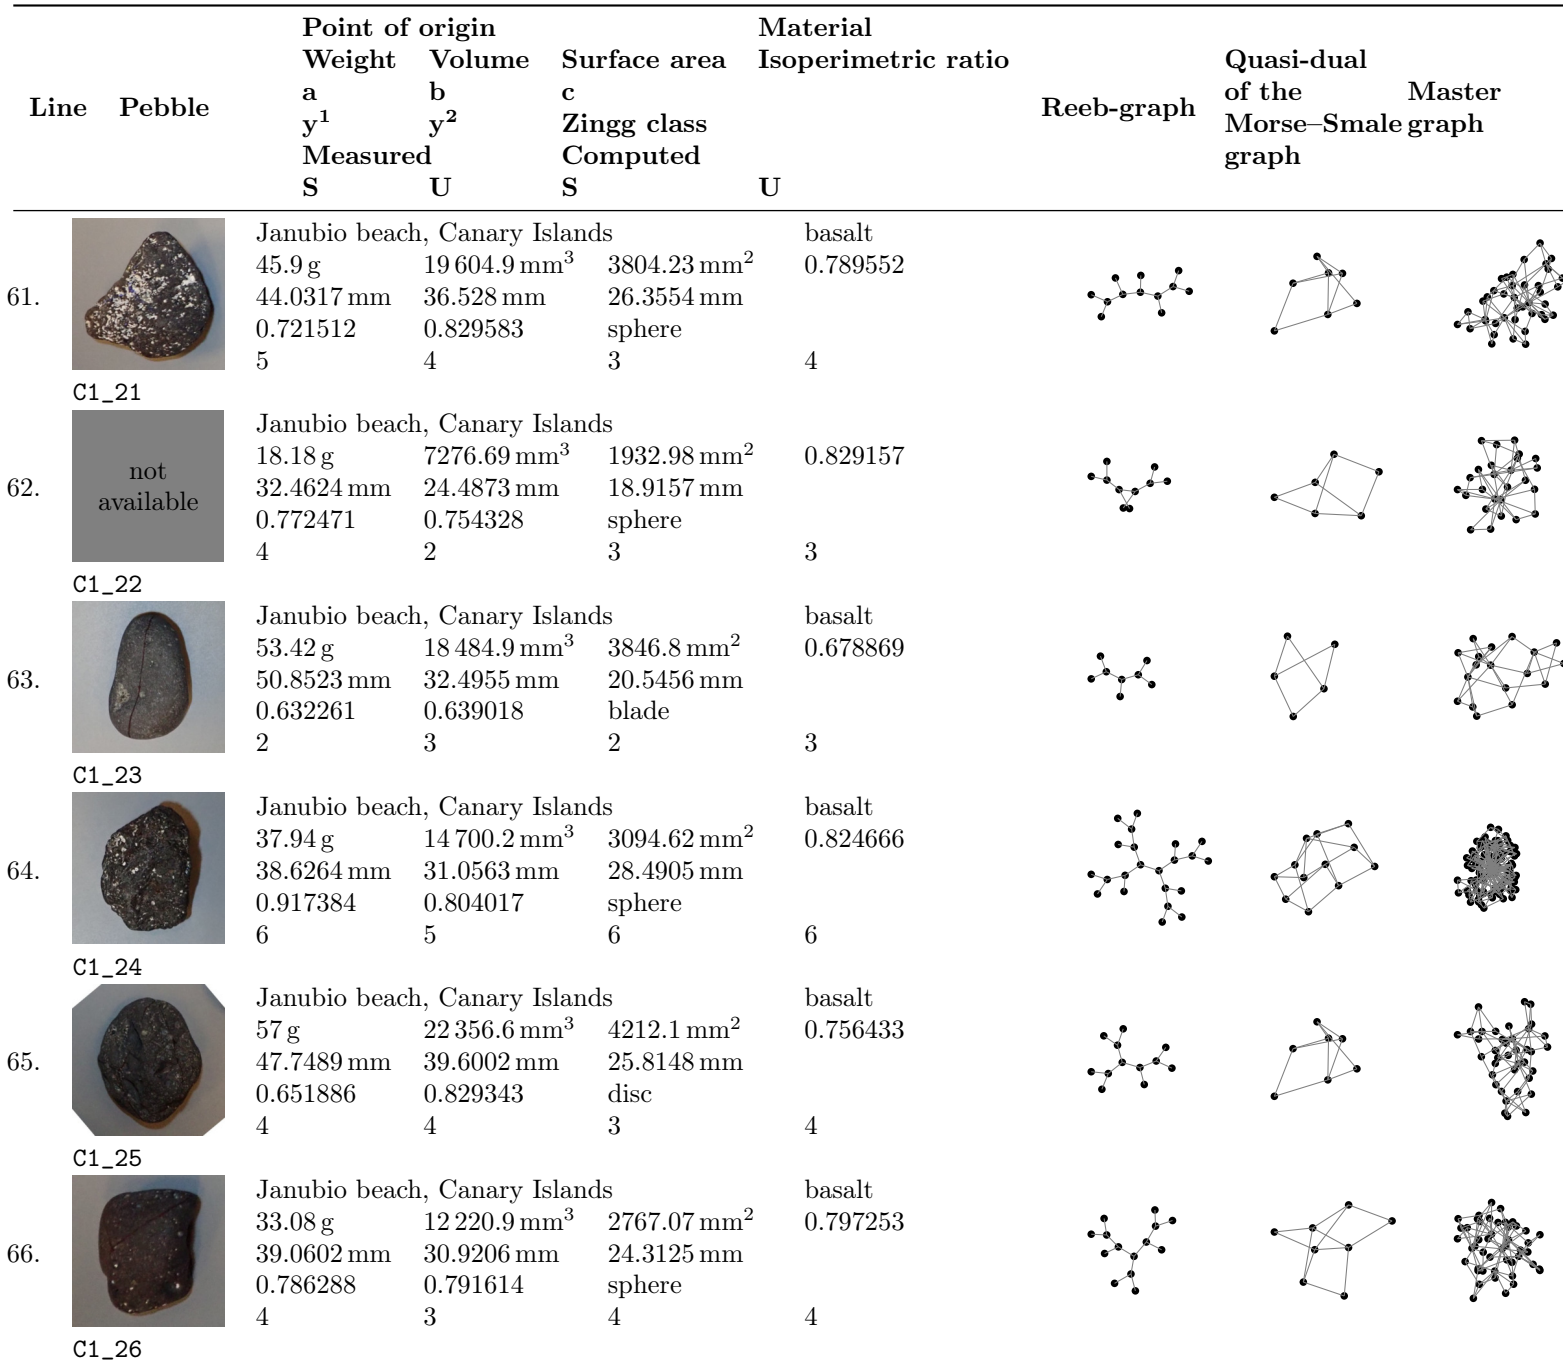  | Janubio beach, Canary Islands |                          |                         | basalt   | 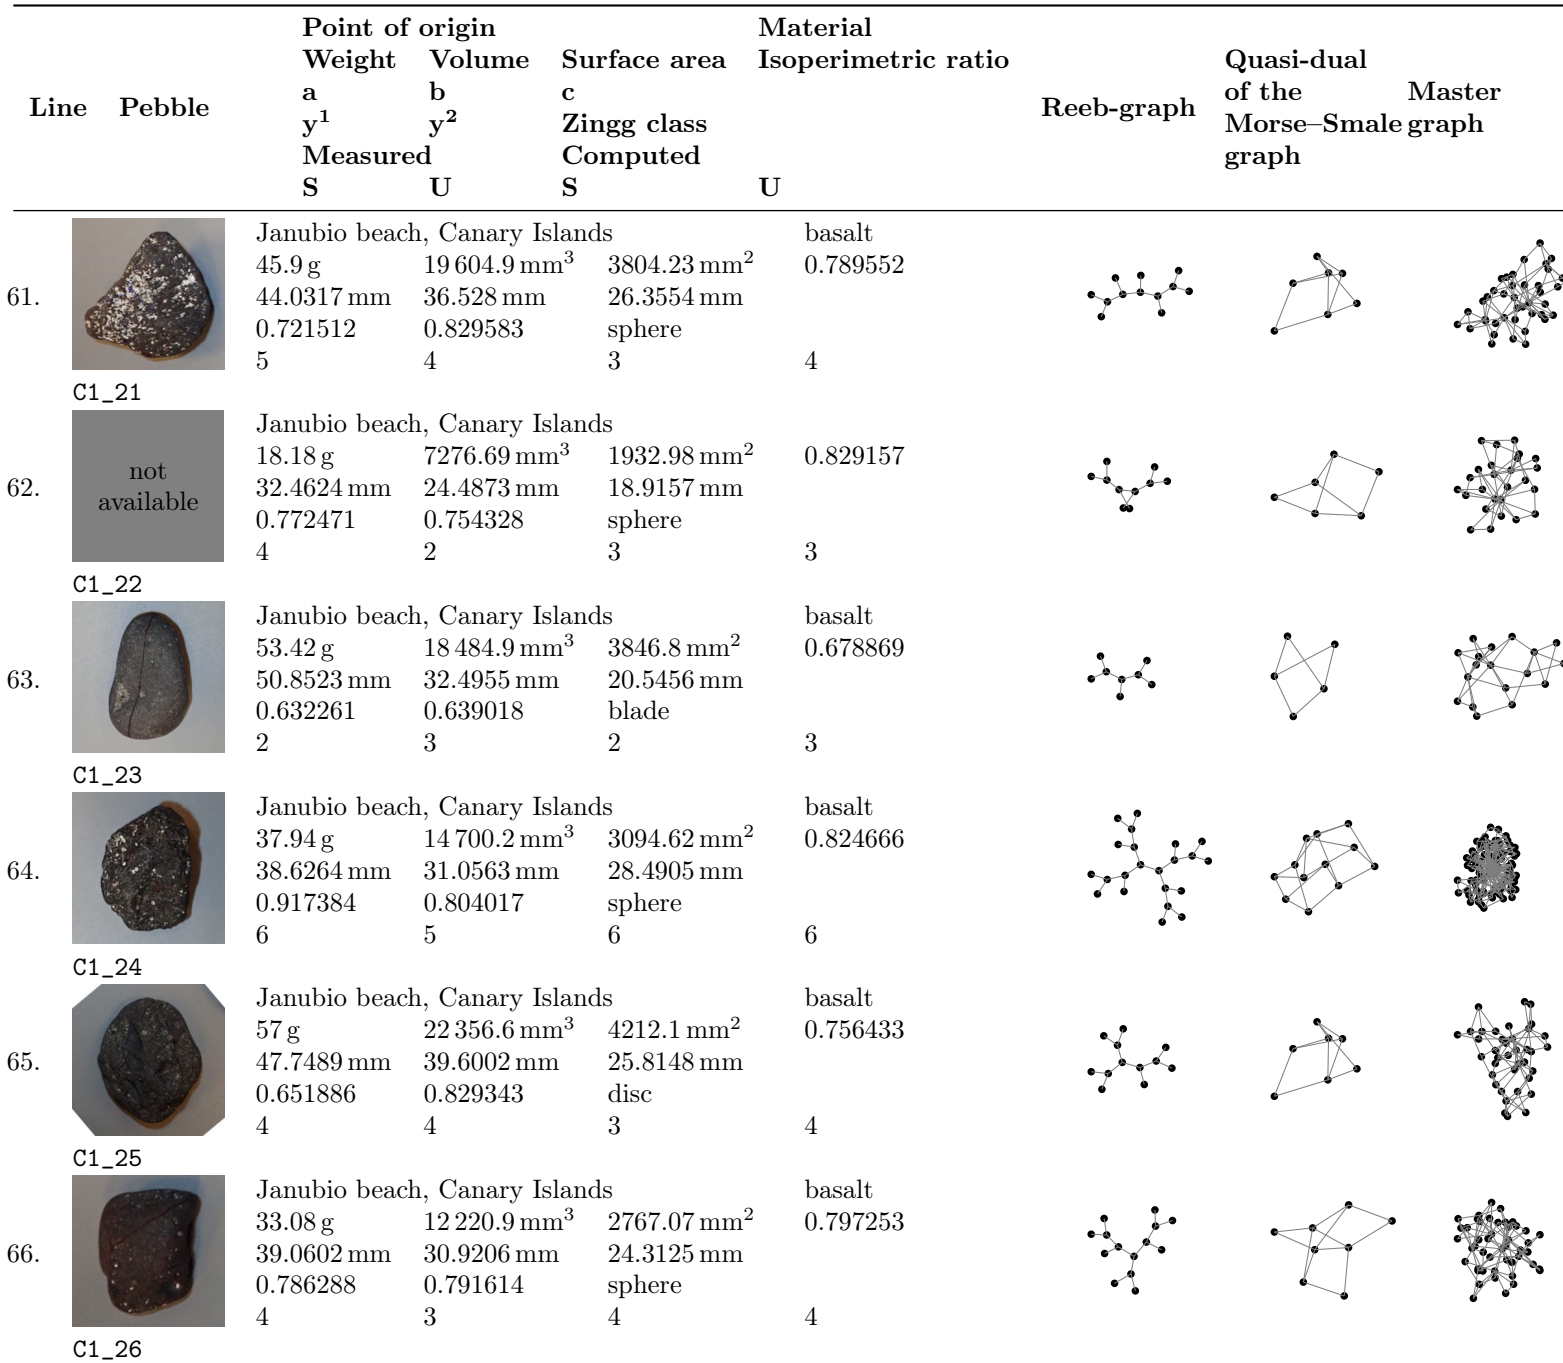  | 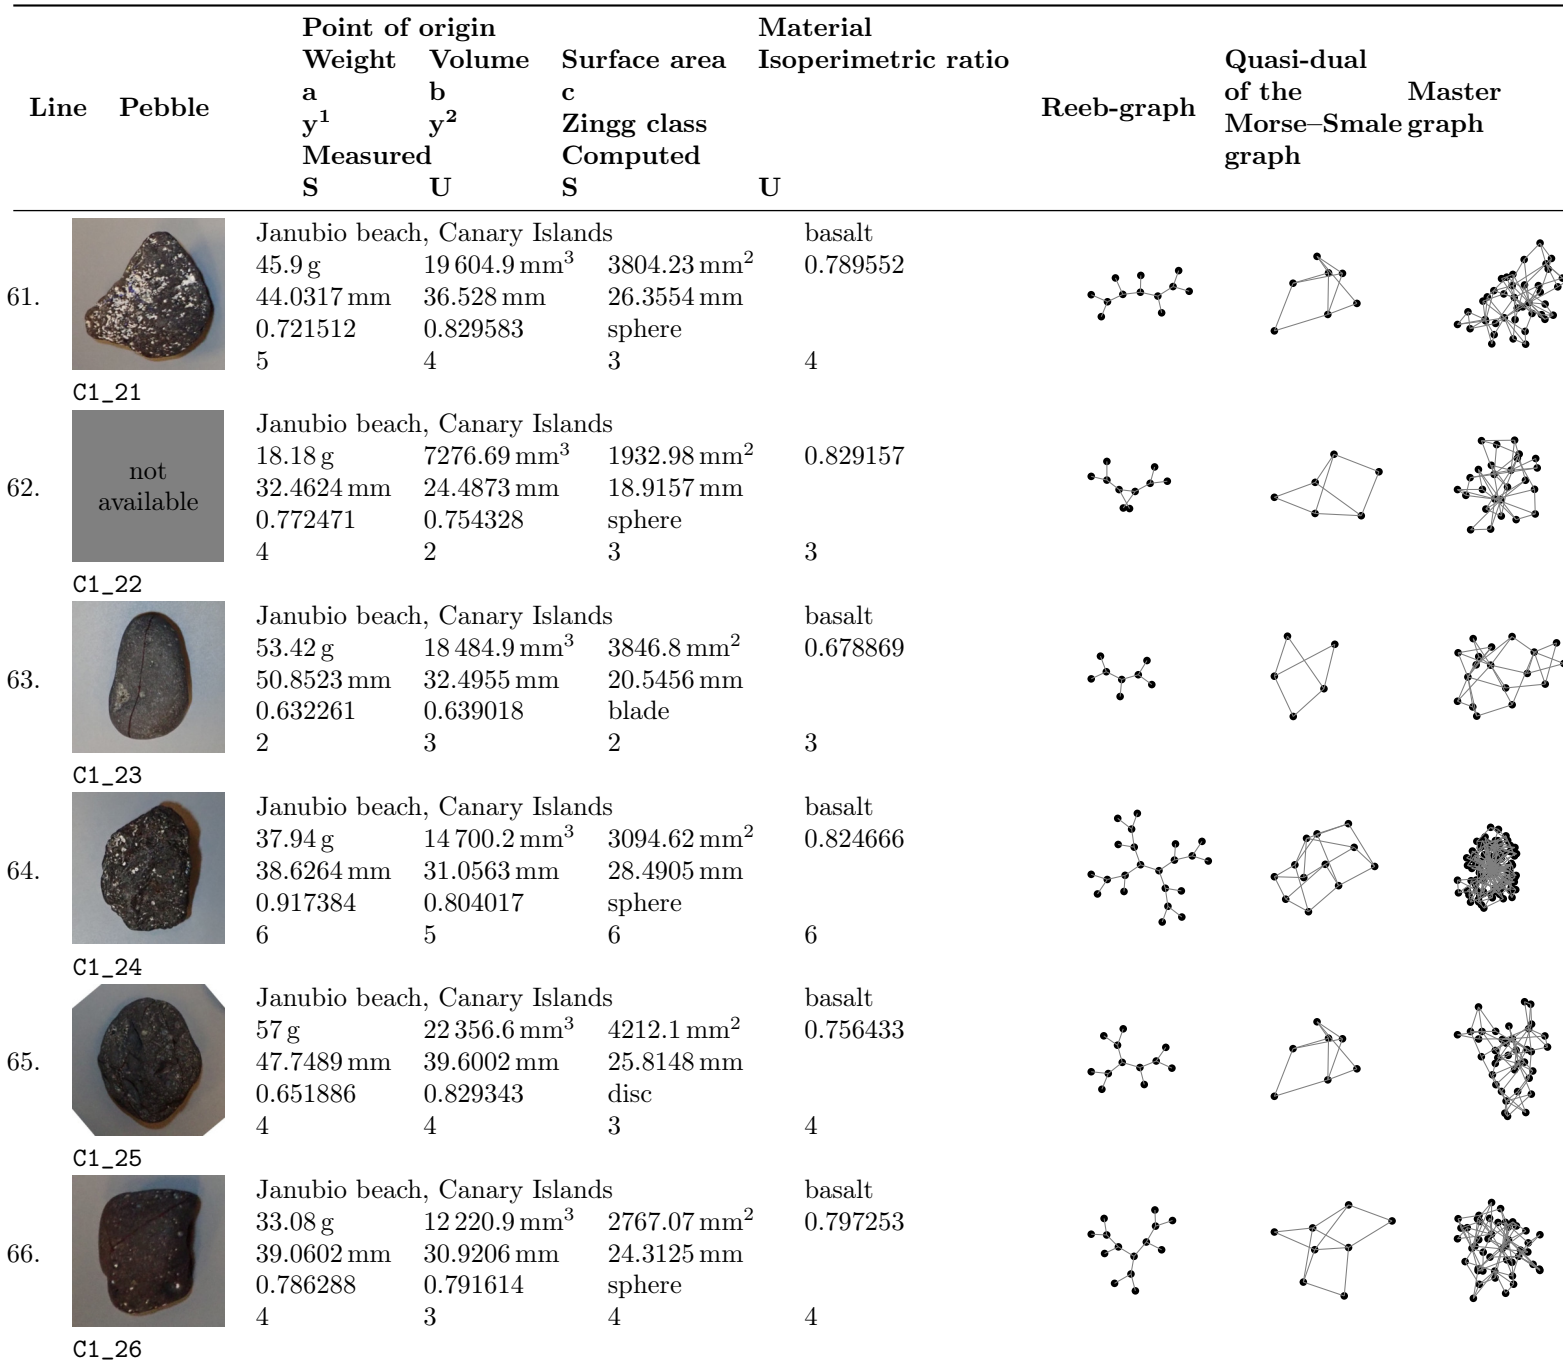  | 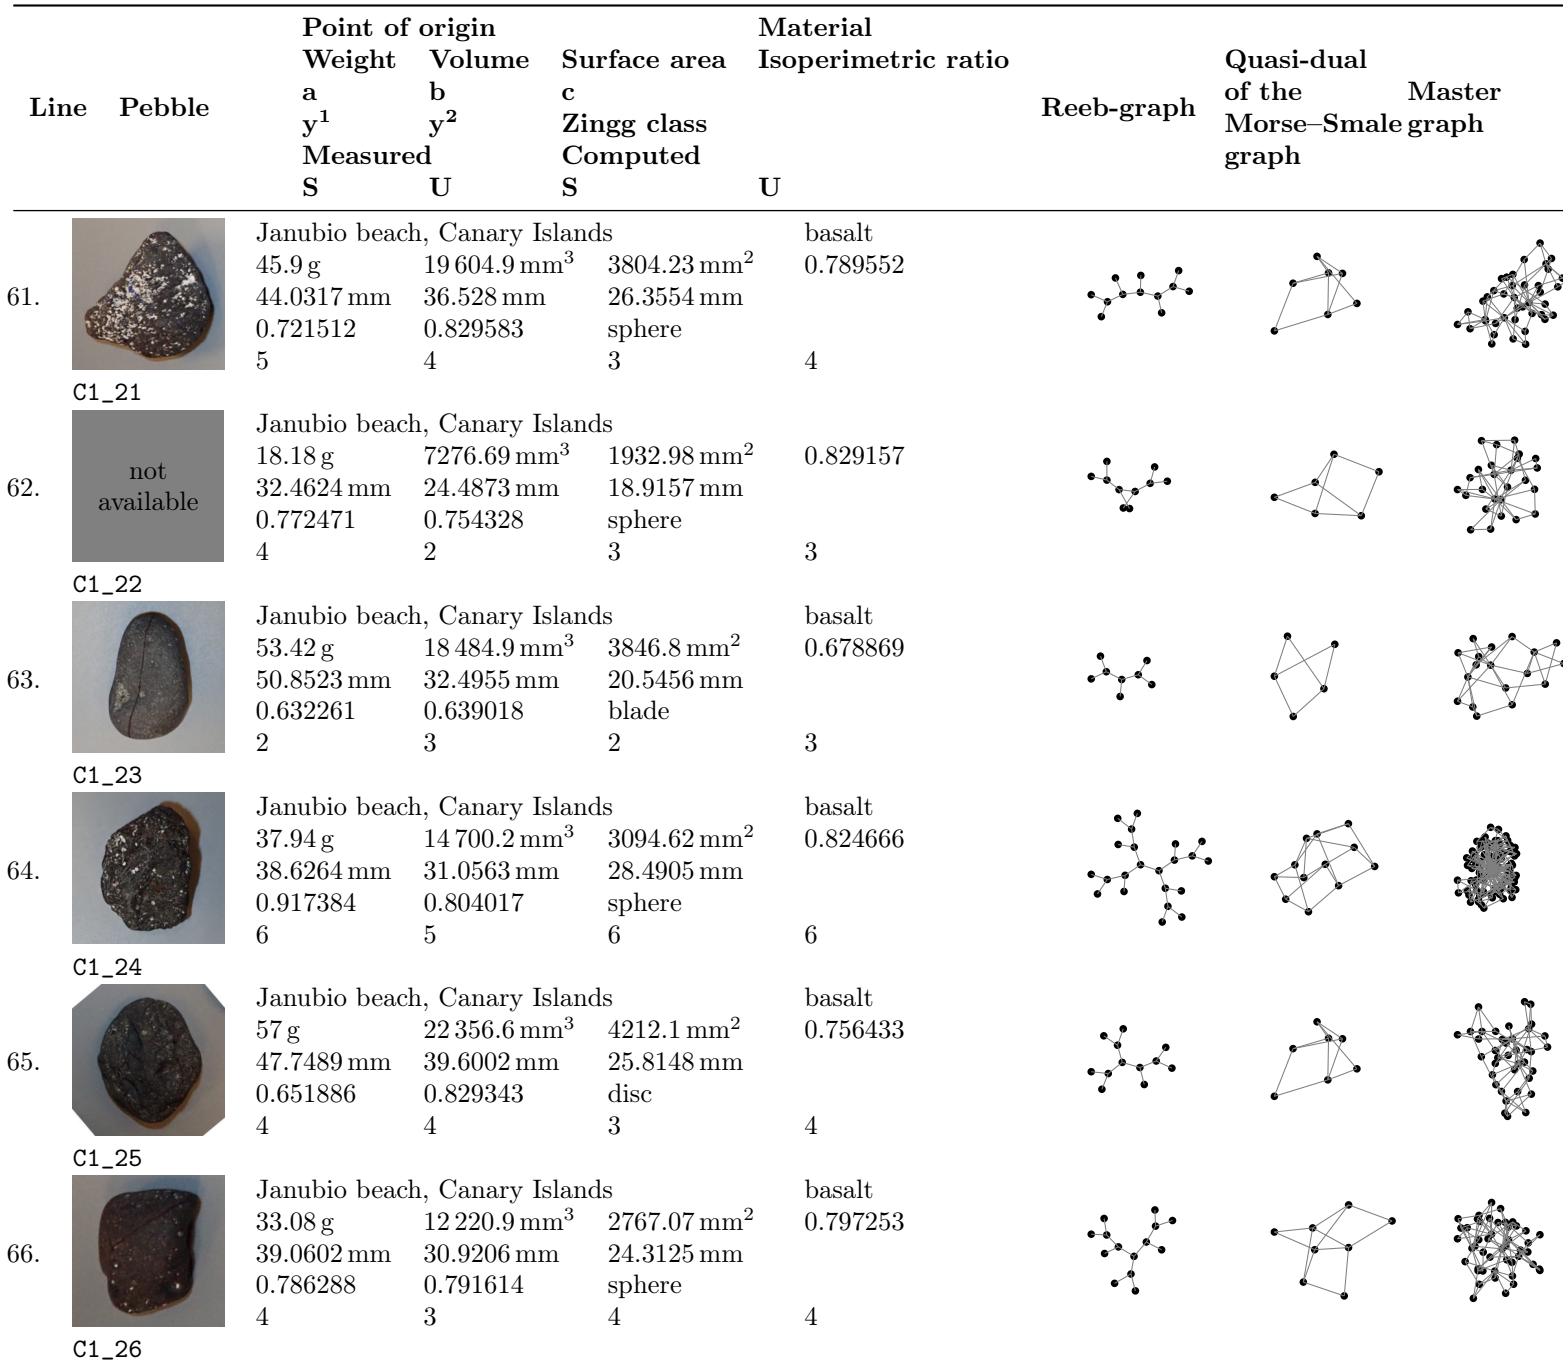  |                 |
|       |                                                                                     | 37.94 g                       | 14 700.2 mm <sup>3</sup> | 3094.62 mm <sup>2</sup> | 0.824666 |                                                                                       |                                                                                       |                                                                                       |                 |
|       |                                                                                     | 38.6264 mm                    | 31.0563 mm               | 28.4905 mm              |          |                                                                                       |                                                                                       |                                                                                       |                 |
|       |                                                                                     | 0.917384                      | 0.804017                 | sphere                  |          |                                                                                       |                                                                                       |                                                                                       |                 |
|       |                                                                                     | 6                             | 5                        | 6                       | 6        |                                                                                       |                                                                                       |                                                                                       |                 |
| C1_24 |                                                                                     |                               |                          |                         |          |                                                                                       |                                                                                       |                                                                                       |                 |
| 65.   | 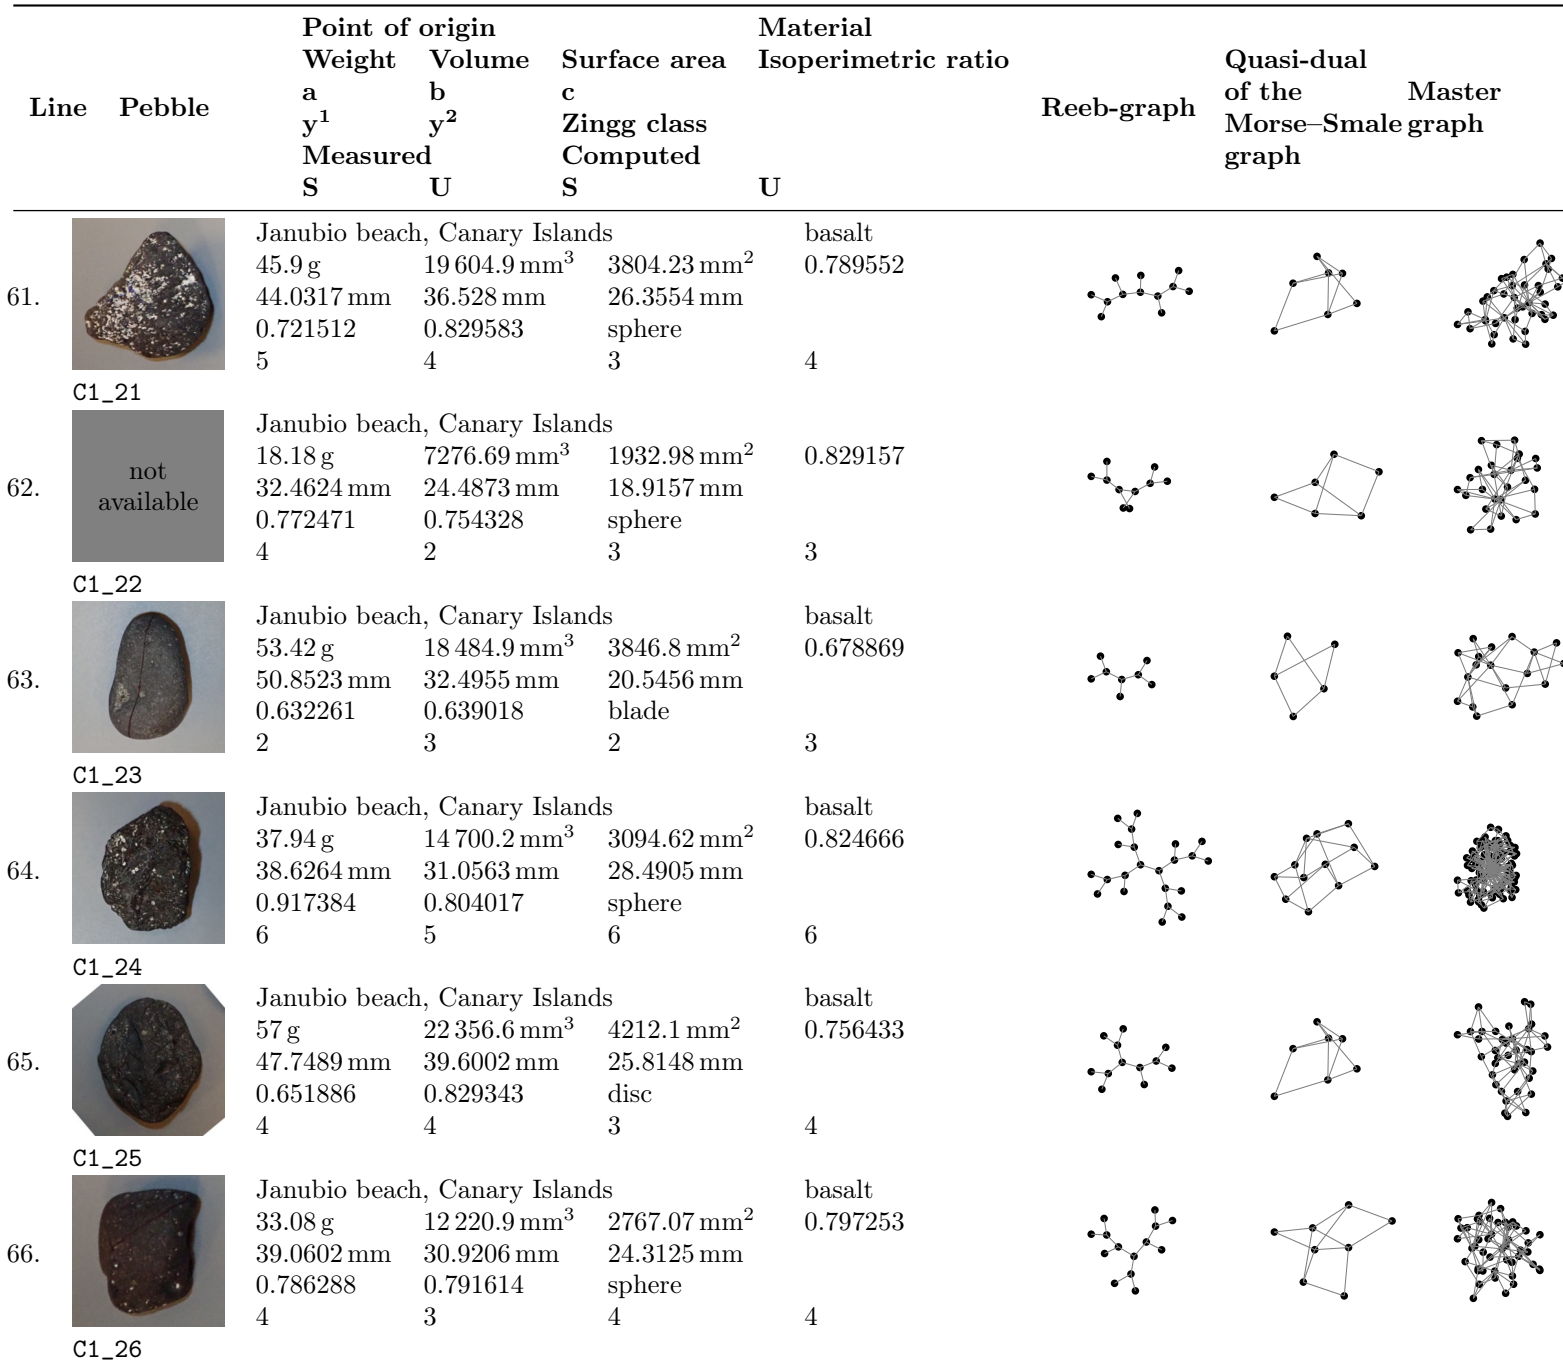 | Janubio beach, Canary Islands |                          |                         | basalt   | 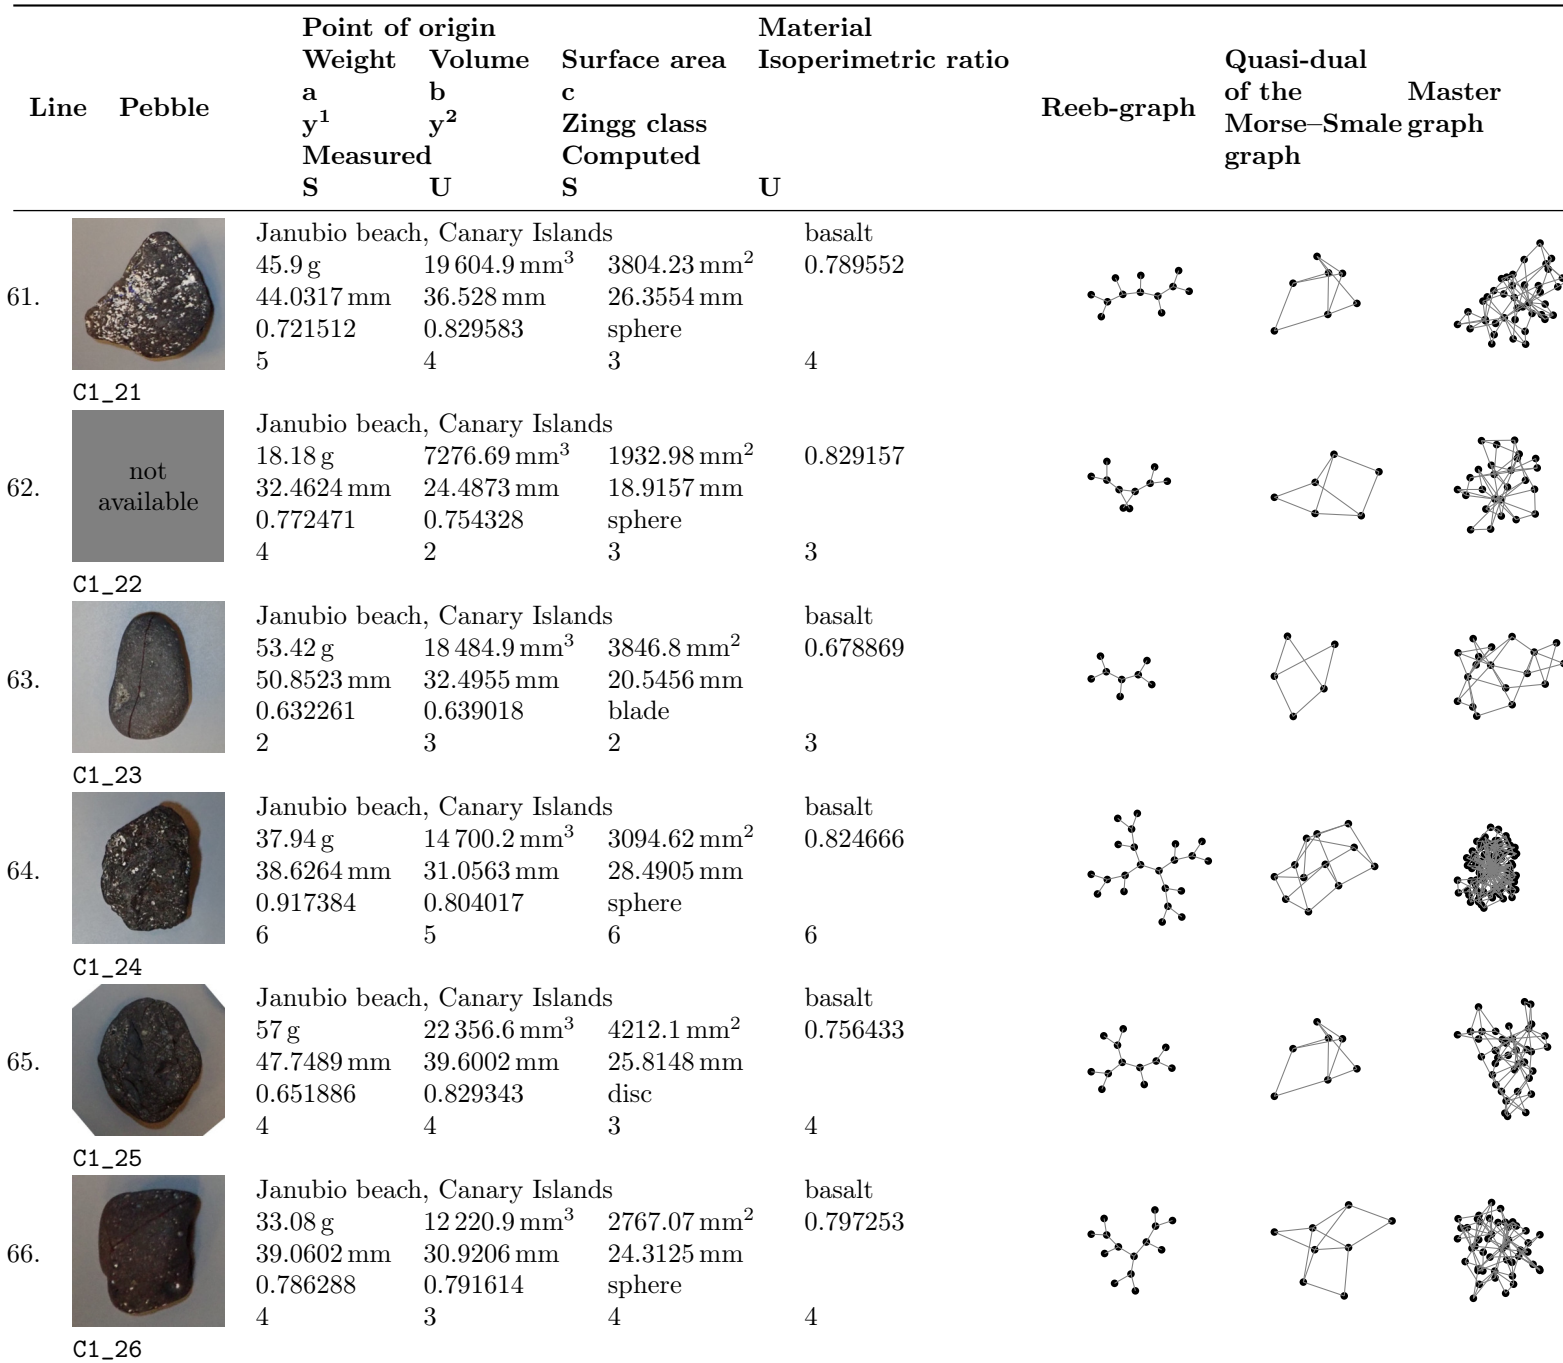 | 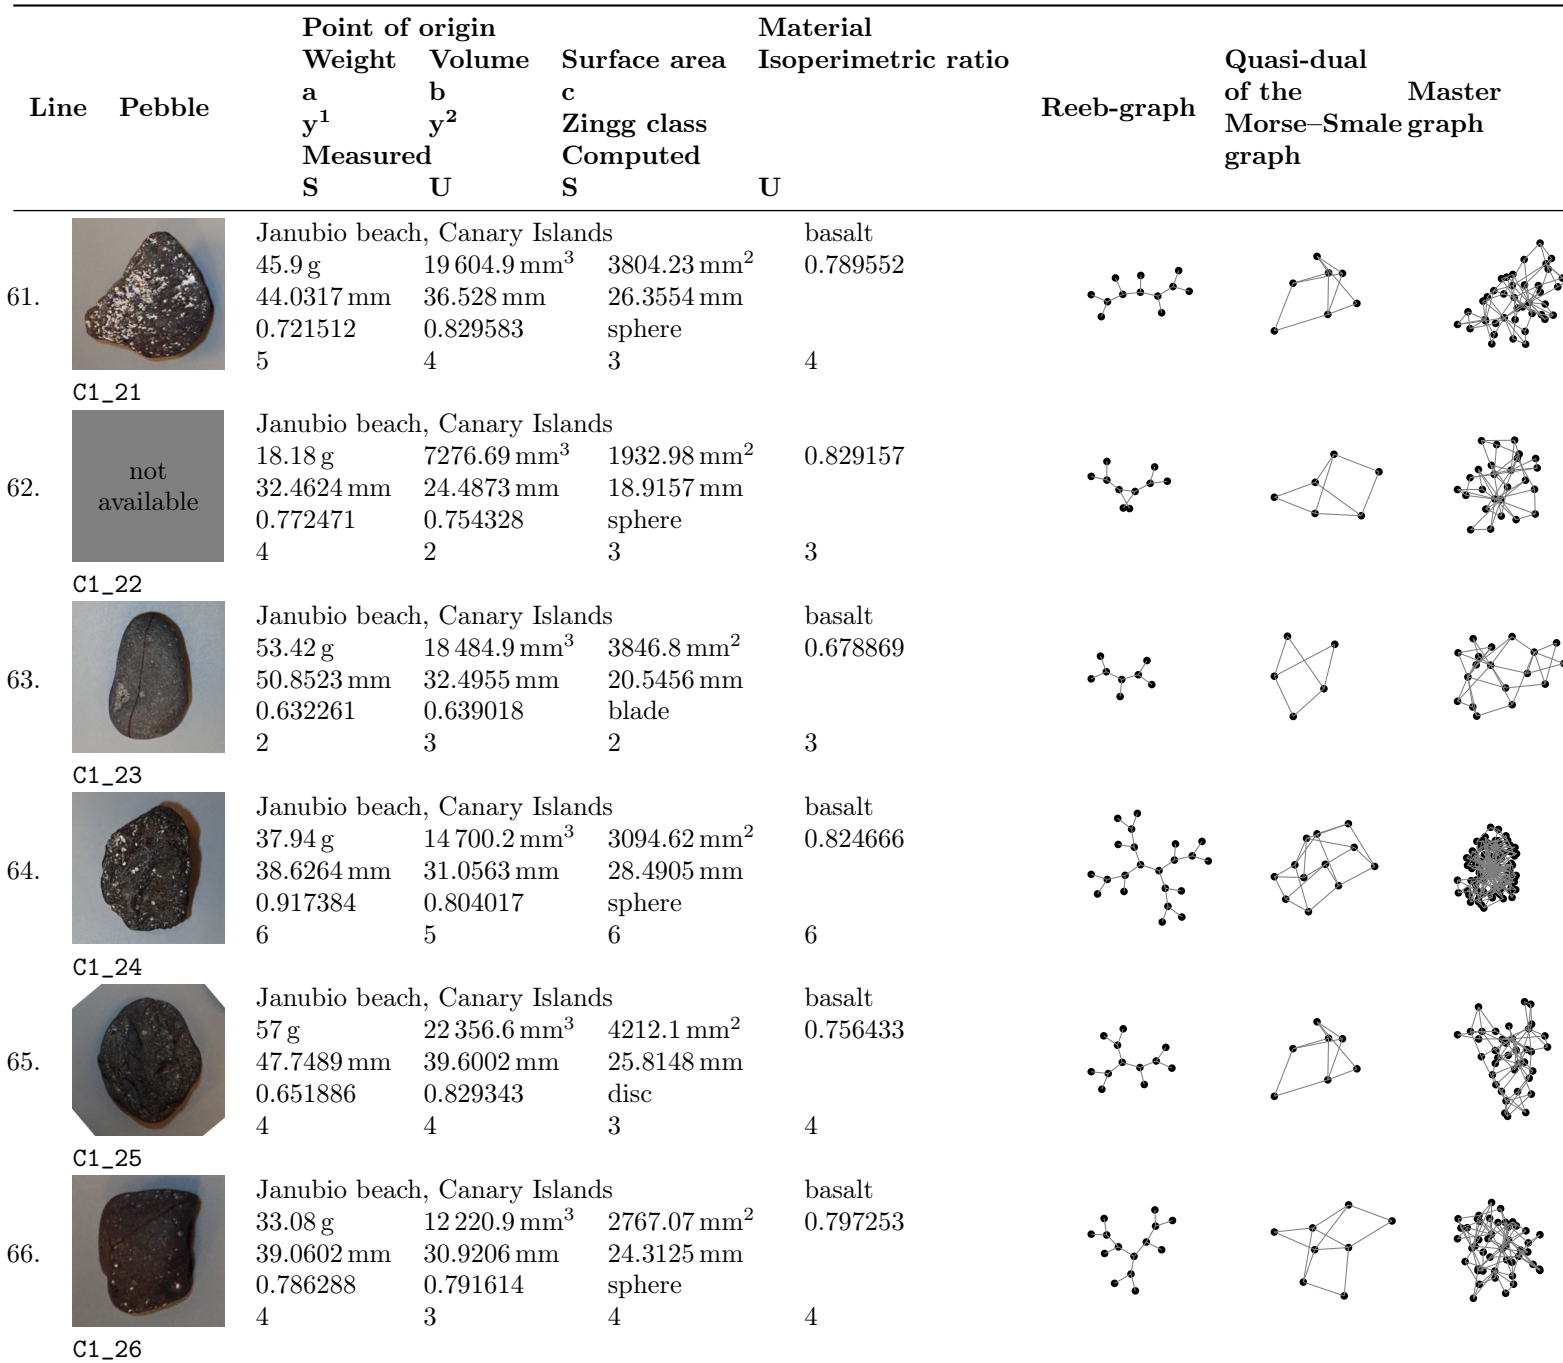 | 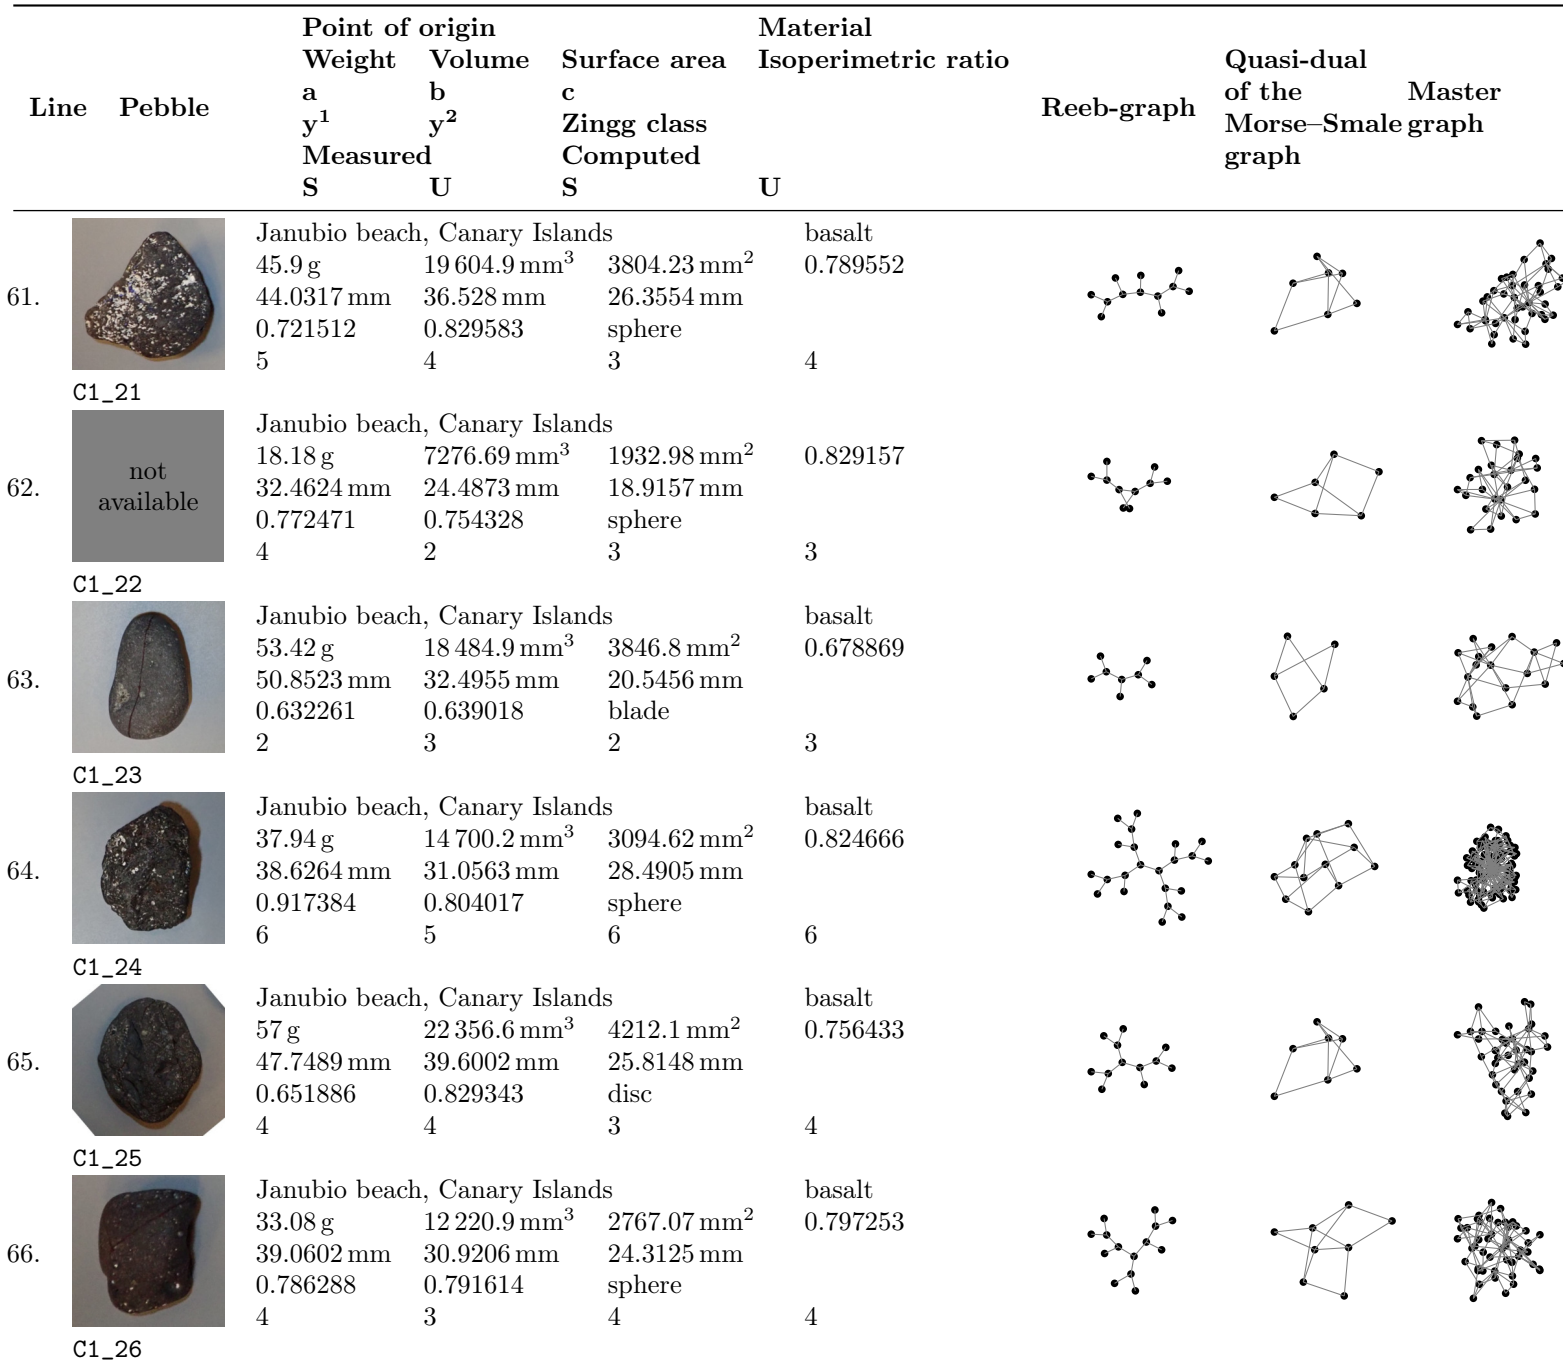 |                 |
|       |                                                                                     | 57 g                          | 22 356.6 mm <sup>3</sup> | 4212.1 mm <sup>2</sup>  | 0.756433 |                                                                                       |                                                                                       |                                                                                       |                 |
|       |                                                                                     | 47.7489 mm                    | 39.6002 mm               | 25.8148 mm              |          |                                                                                       |                                                                                       |                                                                                       |                 |
|       |                                                                                     | 0.651886                      | 0.829343                 | disc                    |          |                                                                                       |                                                                                       |                                                                                       |                 |
|       |                                                                                     | 4                             | 4                        | 3                       | 4        |                                                                                       |                                                                                       |                                                                                       |                 |
| C1_25 |                                                                                     |                               |                          |                         |          |                                                                                       |                                                                                       |                                                                                       |                 |
| 66.   | 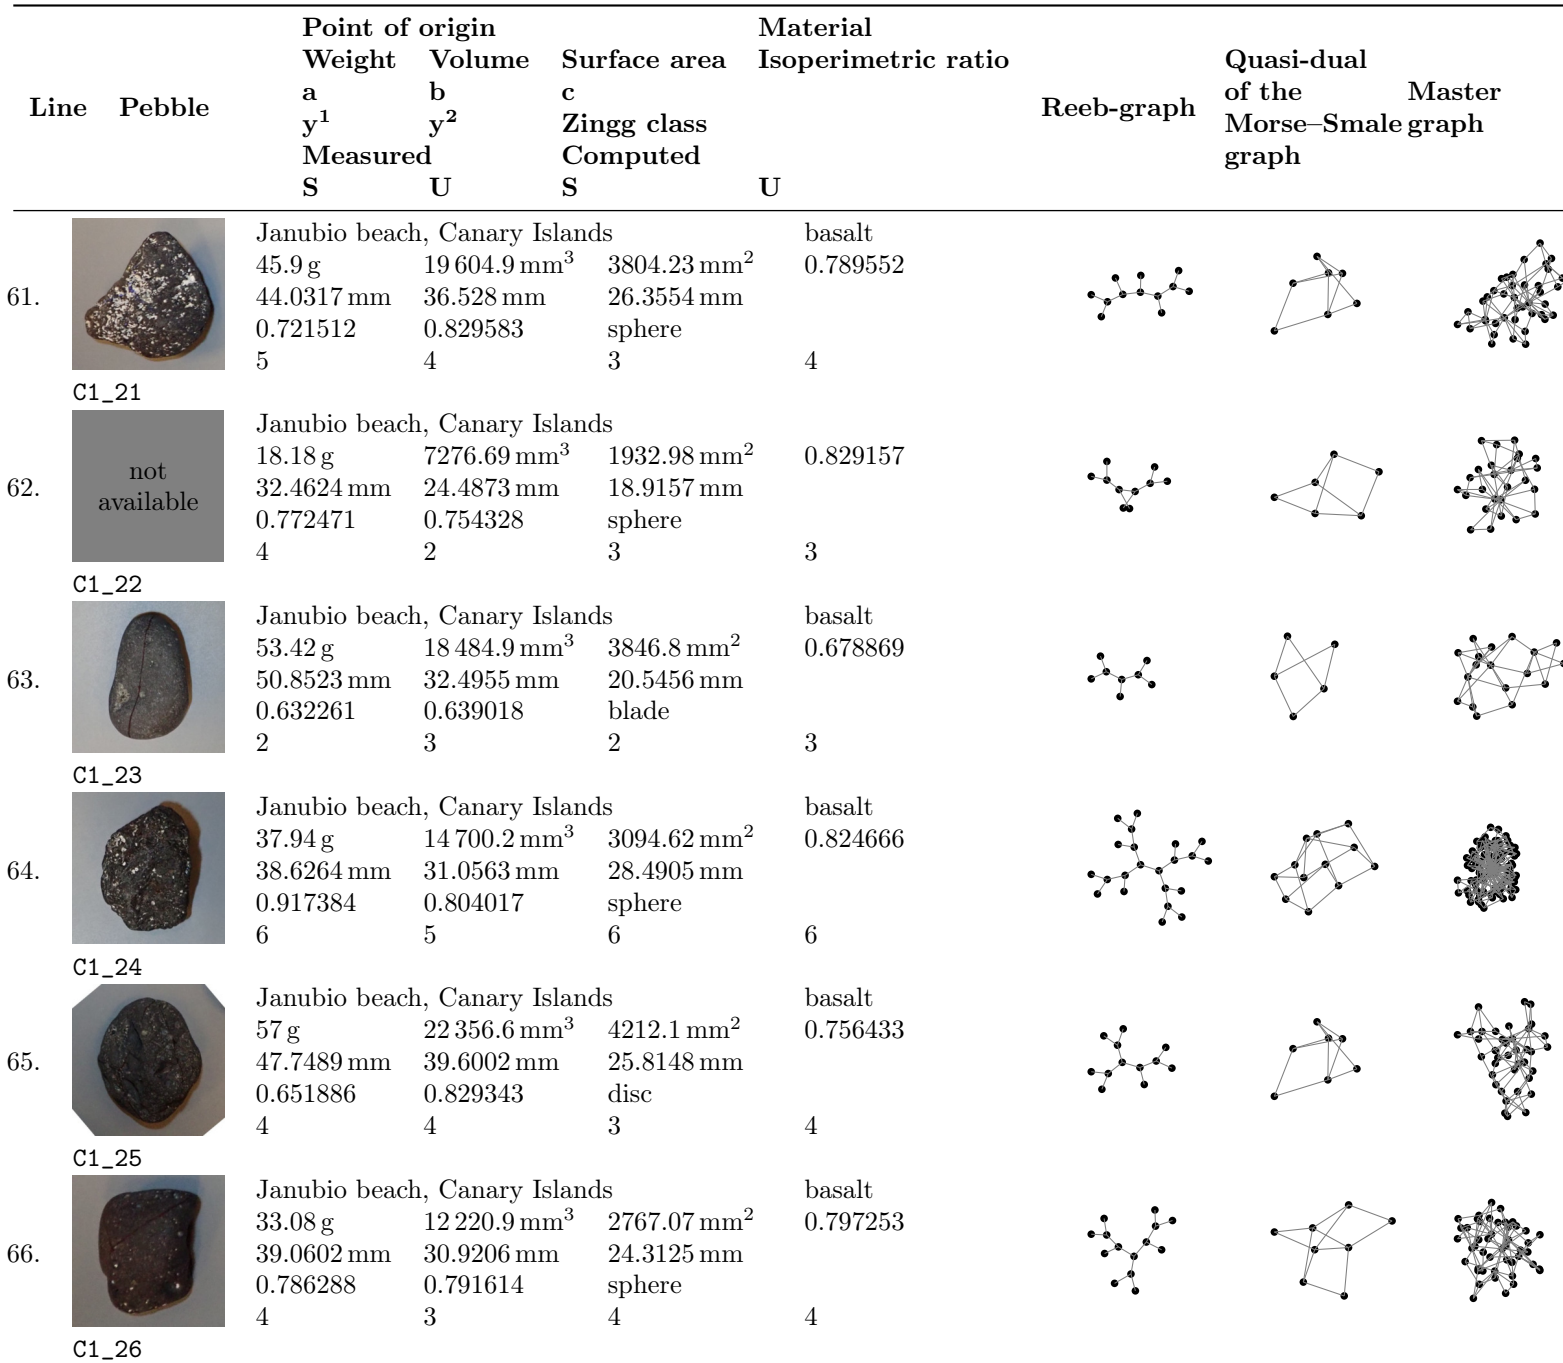 | Janubio beach, Canary Islands |                          |                         | basalt   | 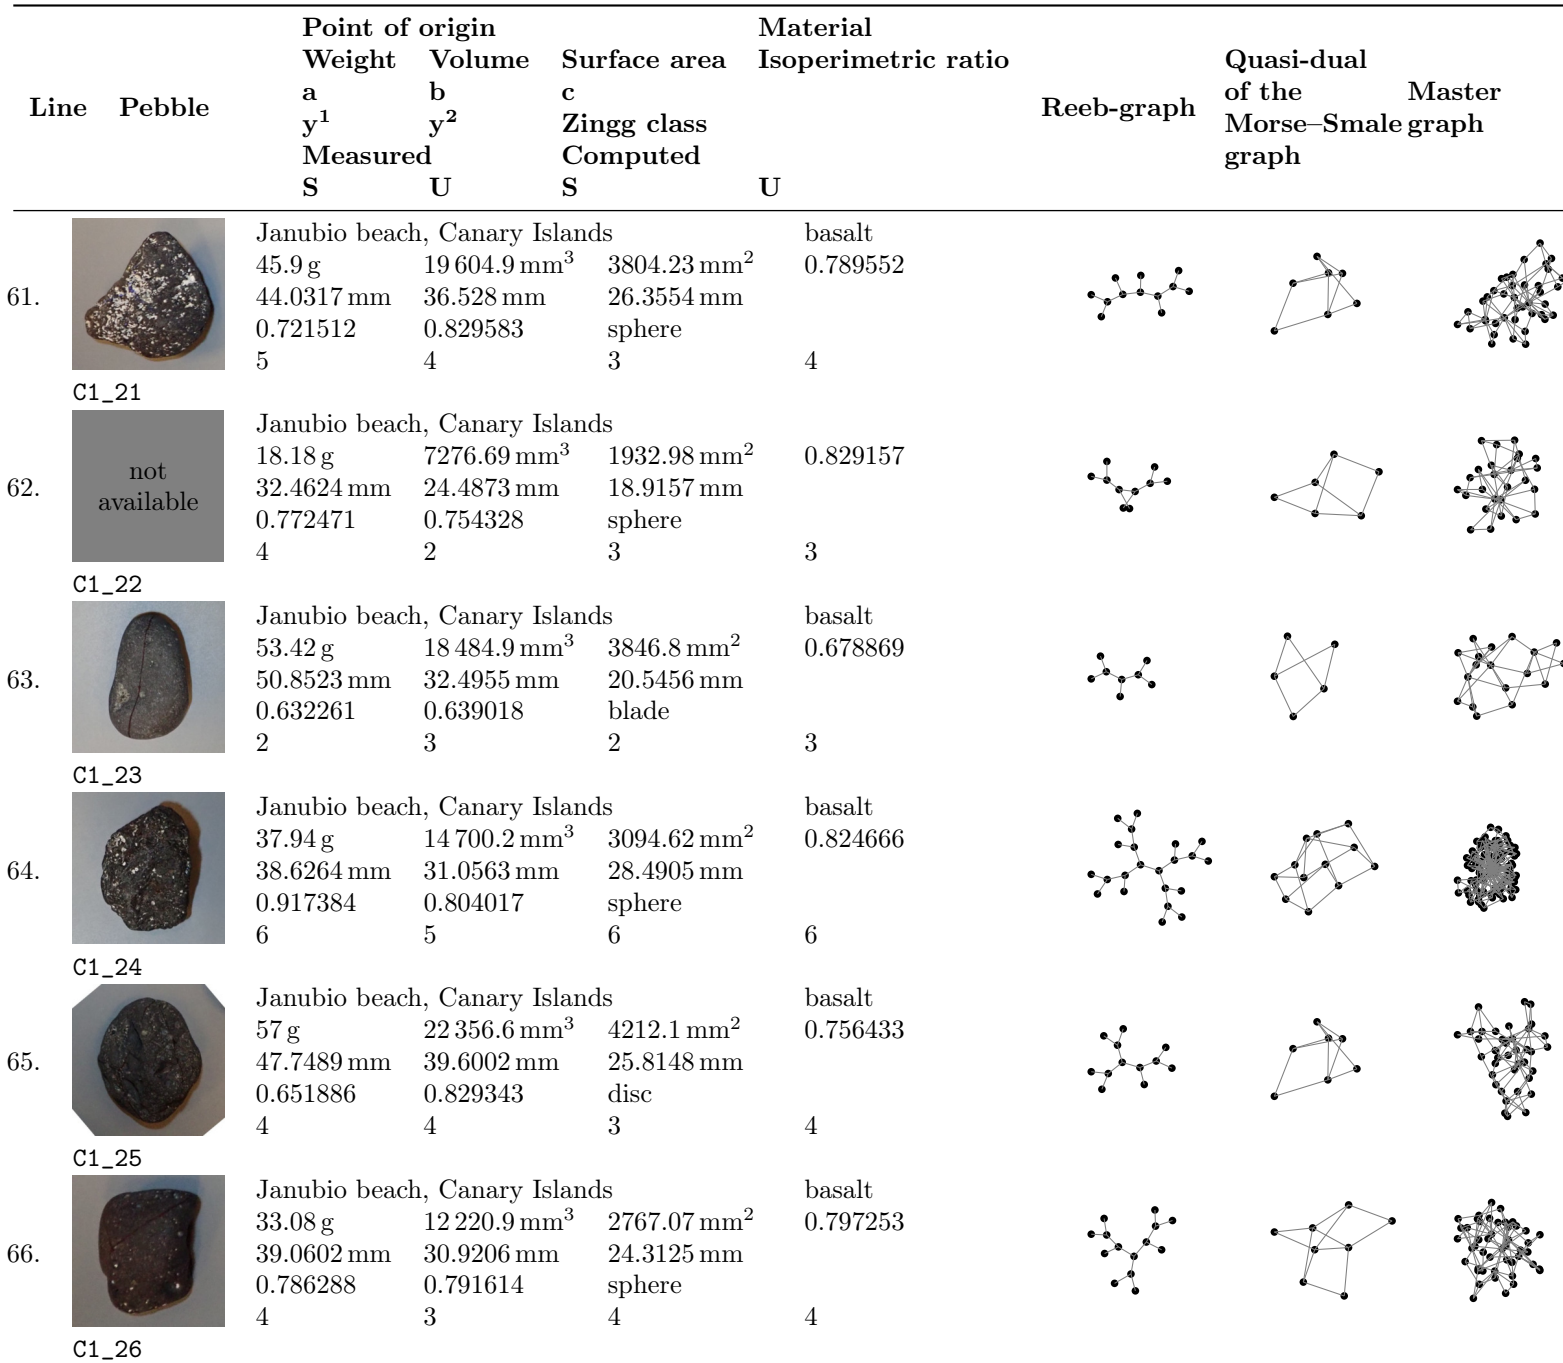 | 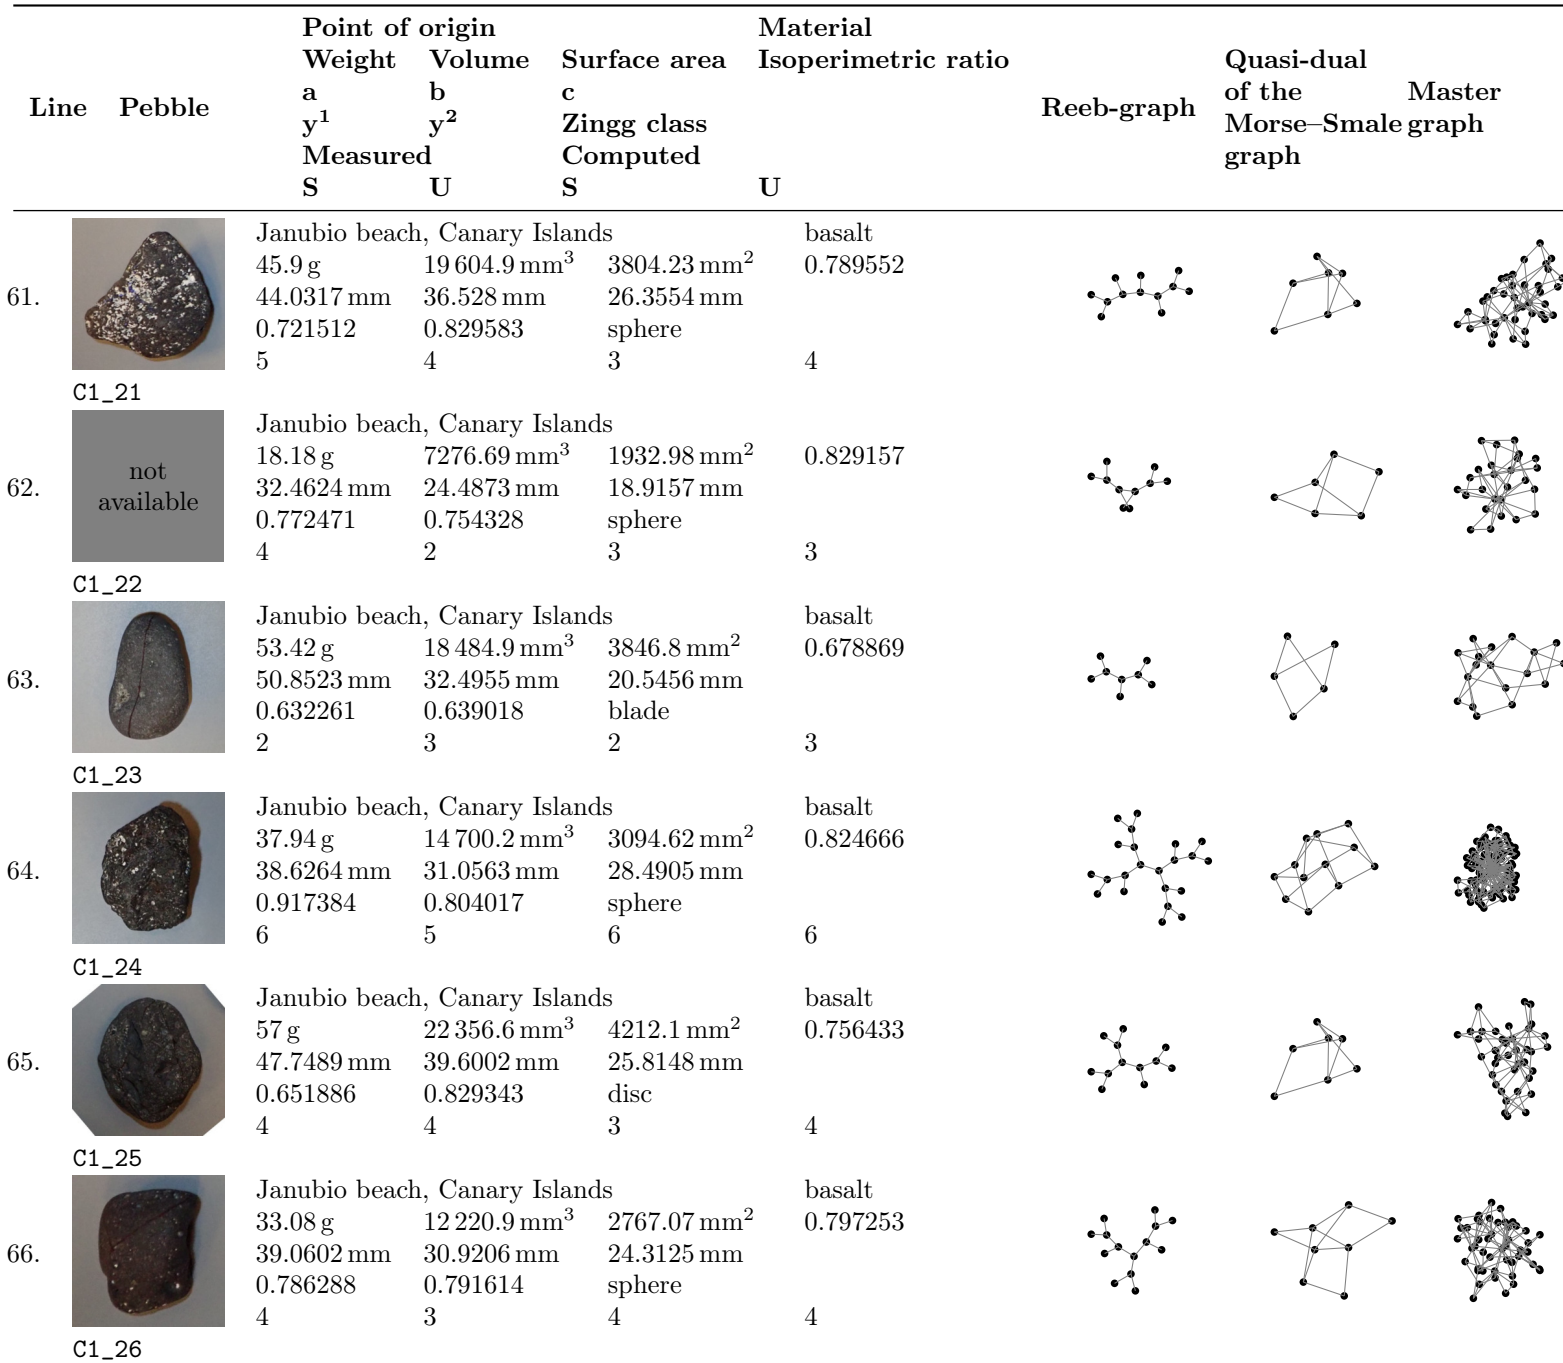 | 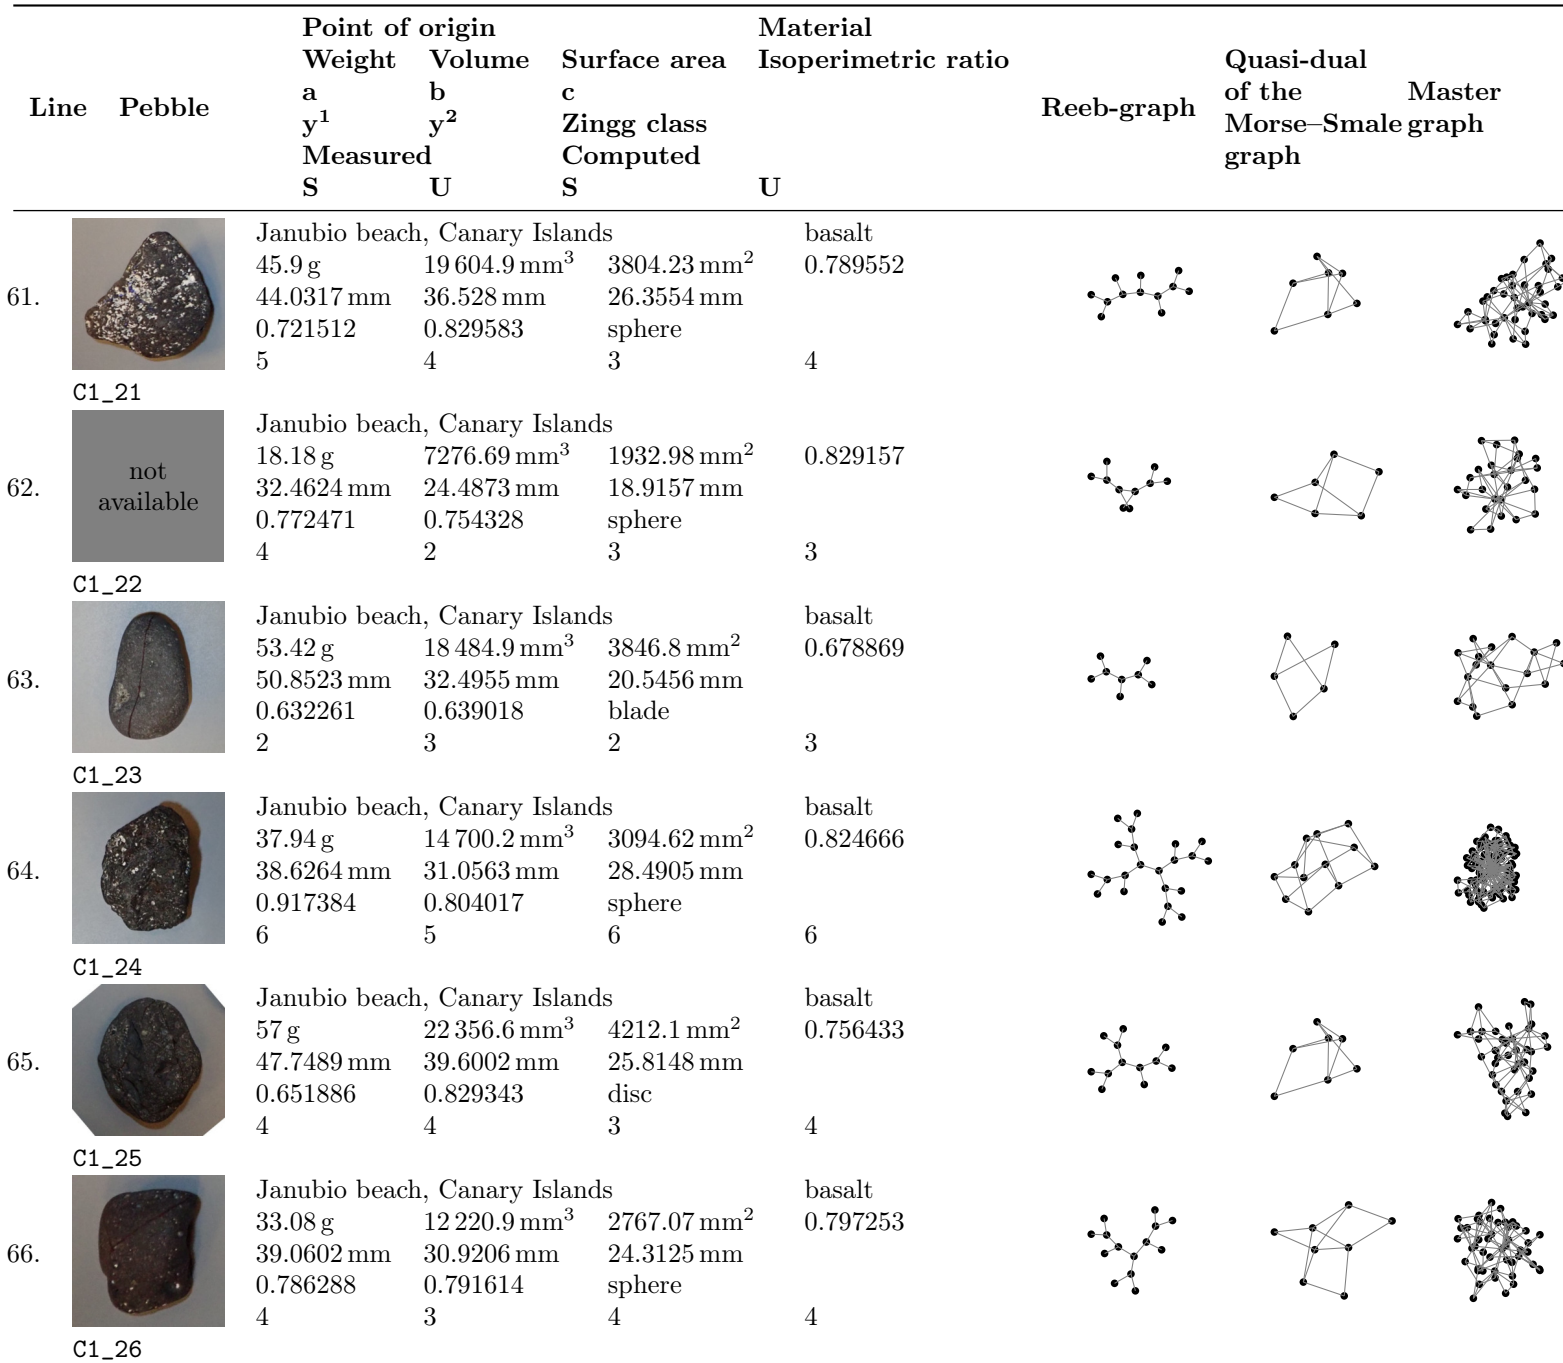 |                 |
|       |                                                                                     | 33.08 g                       | 12 220.9 mm <sup>3</sup> | 2767.07 mm <sup>2</sup> | 0.797253 |                                                                                       |                                                                                       |                                                                                       |                 |
|       |                                                                                     | 39.0602 mm                    | 30.9206 mm               | 24.3125 mm              |          |                                                                                       |                                                                                       |                                                                                       |                 |
|       |                                                                                     | 0.786288                      | 0.791614                 | sphere                  |          |                                                                                       |                                                                                       |                                                                                       |                 |
|       |                                                                                     | 4                             | 3                        | 4                       | 4        |                                                                                       |                                                                                       |                                                                                       |                 |
| C1_26 |                                                                                     |                               |                          |                         |          |                                                                                       |                                                                                       |                                                                                       |                 |

| Line | Pebble                                                                              | Point of origin               |                          |                         | Material | Isoperimetric ratio | Reeb-graph                                                                            | Quasi-dual<br>of the<br>Morse–Smale<br>graph                                          | Master                                                                                |
|------|-------------------------------------------------------------------------------------|-------------------------------|--------------------------|-------------------------|----------|---------------------|---------------------------------------------------------------------------------------|---------------------------------------------------------------------------------------|---------------------------------------------------------------------------------------|
|      |                                                                                     | Weight                        | Volume                   | Surface area            |          |                     |                                                                                       |                                                                                       |                                                                                       |
|      |                                                                                     | a                             | b                        | c                       |          |                     |                                                                                       |                                                                                       |                                                                                       |
|      |                                                                                     | y <sup>1</sup>                | y <sup>2</sup>           | Zingg class             |          |                     |                                                                                       |                                                                                       |                                                                                       |
|      |                                                                                     | Measured                      |                          | Computed                |          |                     |                                                                                       |                                                                                       |                                                                                       |
|      |                                                                                     | S                             | U                        | S                       |          | U                   |                                                                                       |                                                                                       |                                                                                       |
| 67.  | 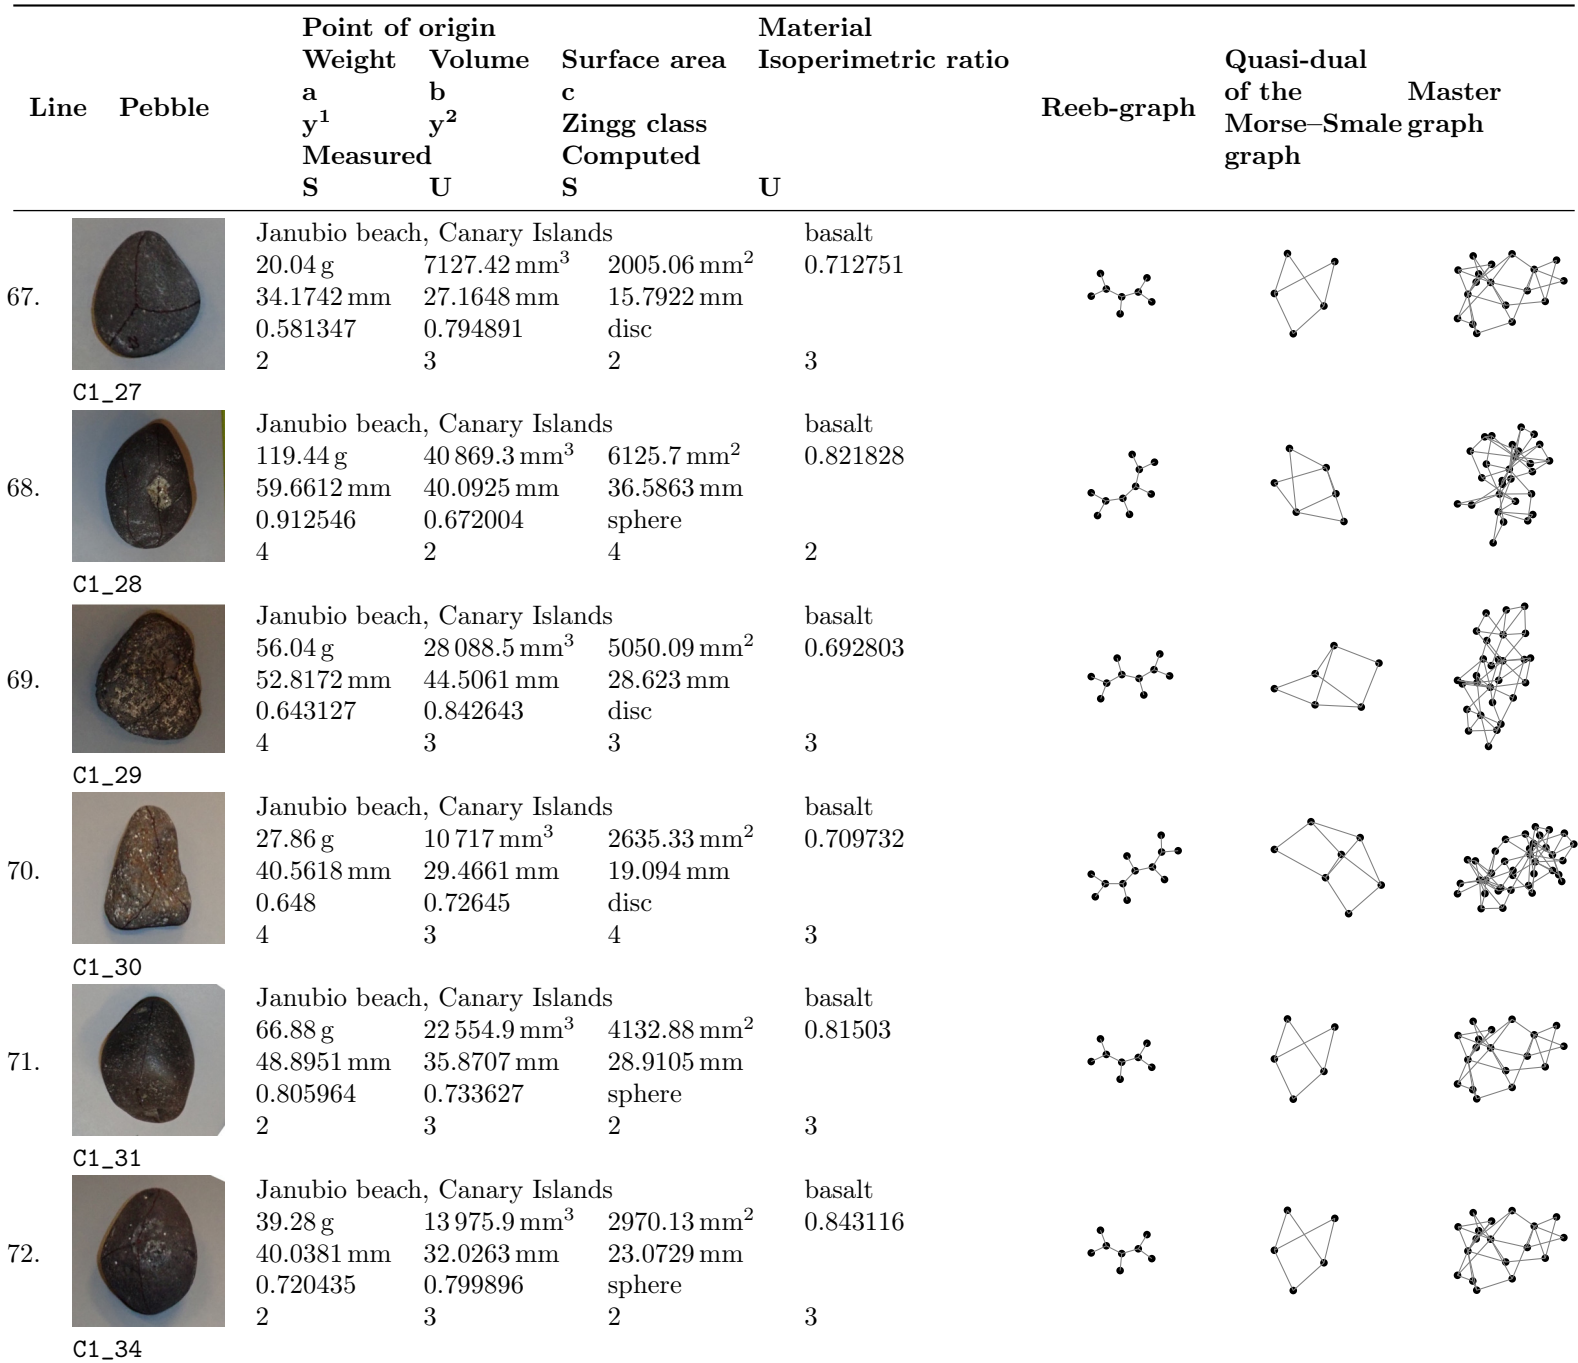   | Janubio beach, Canary Islands |                          |                         | basalt   | 0.712751            | 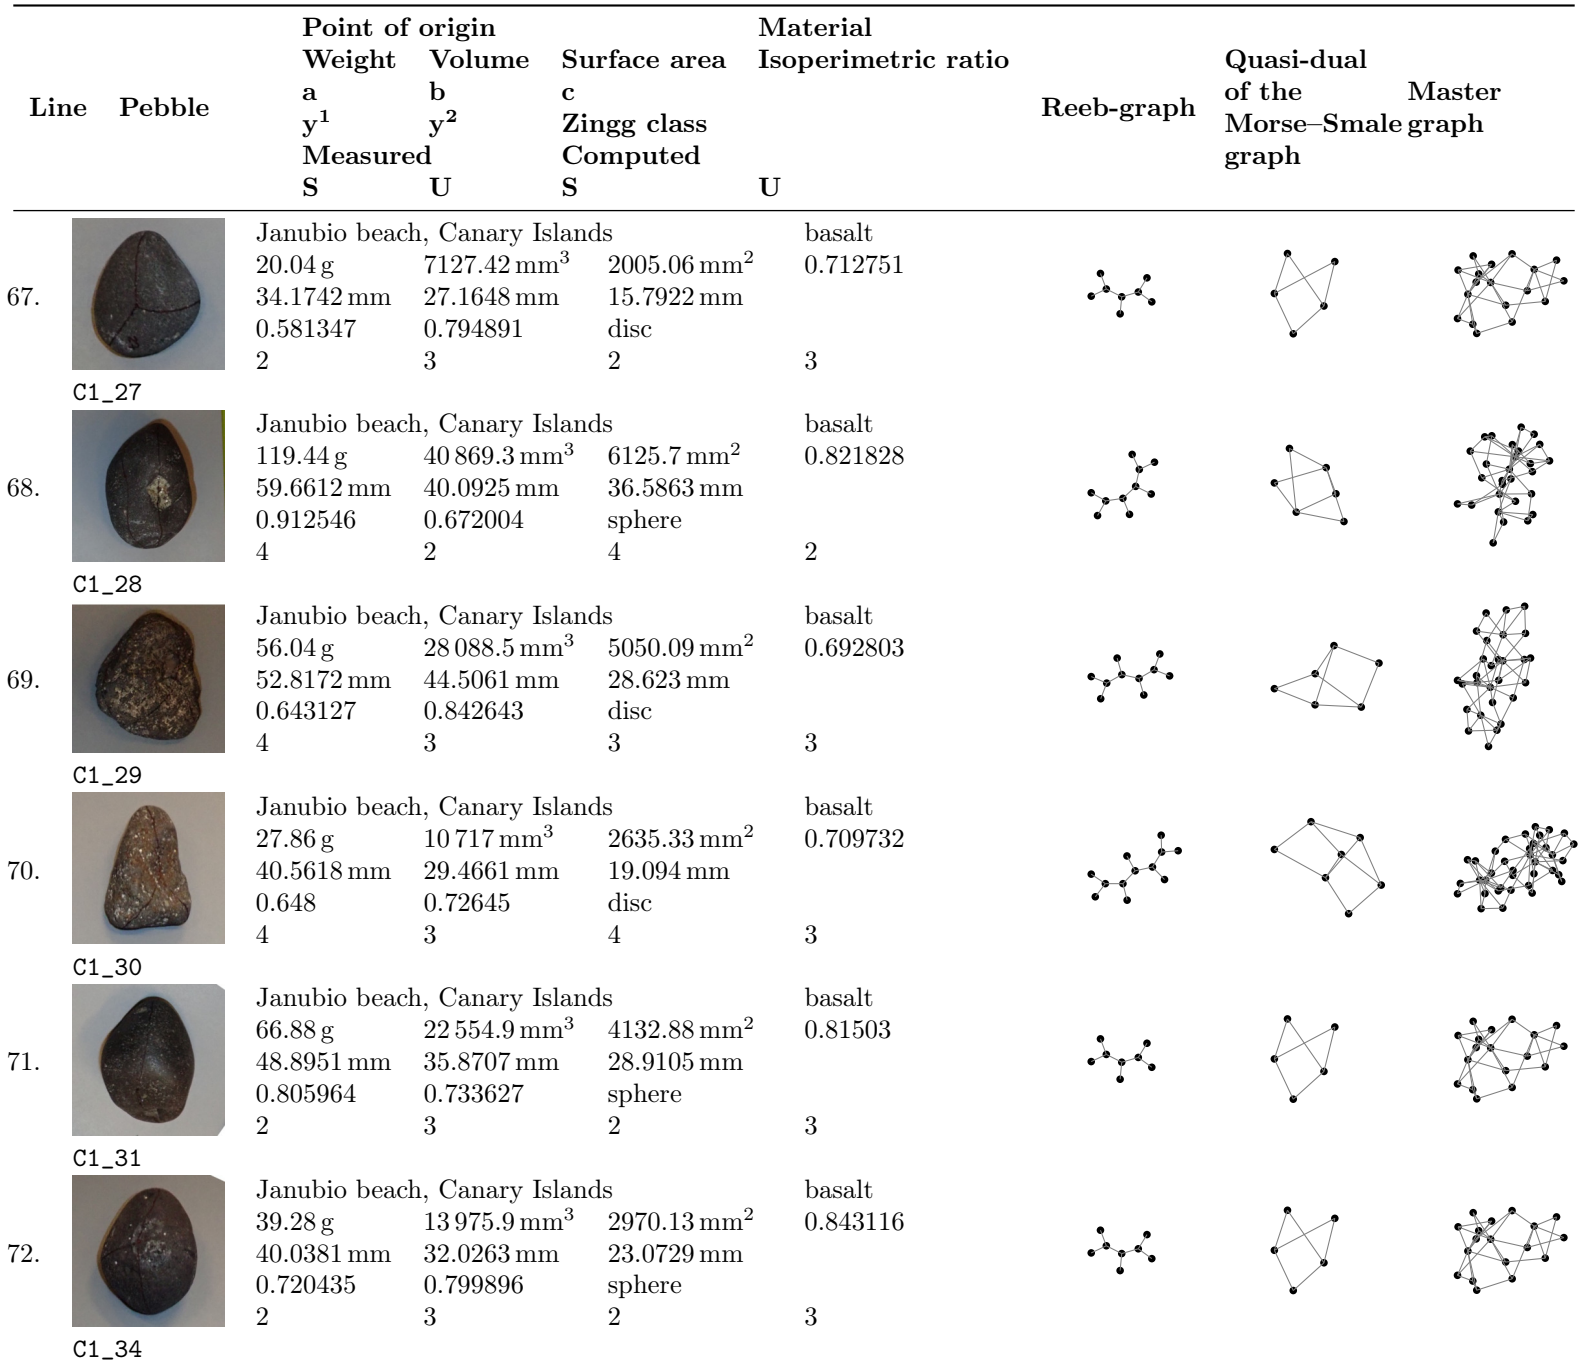   | 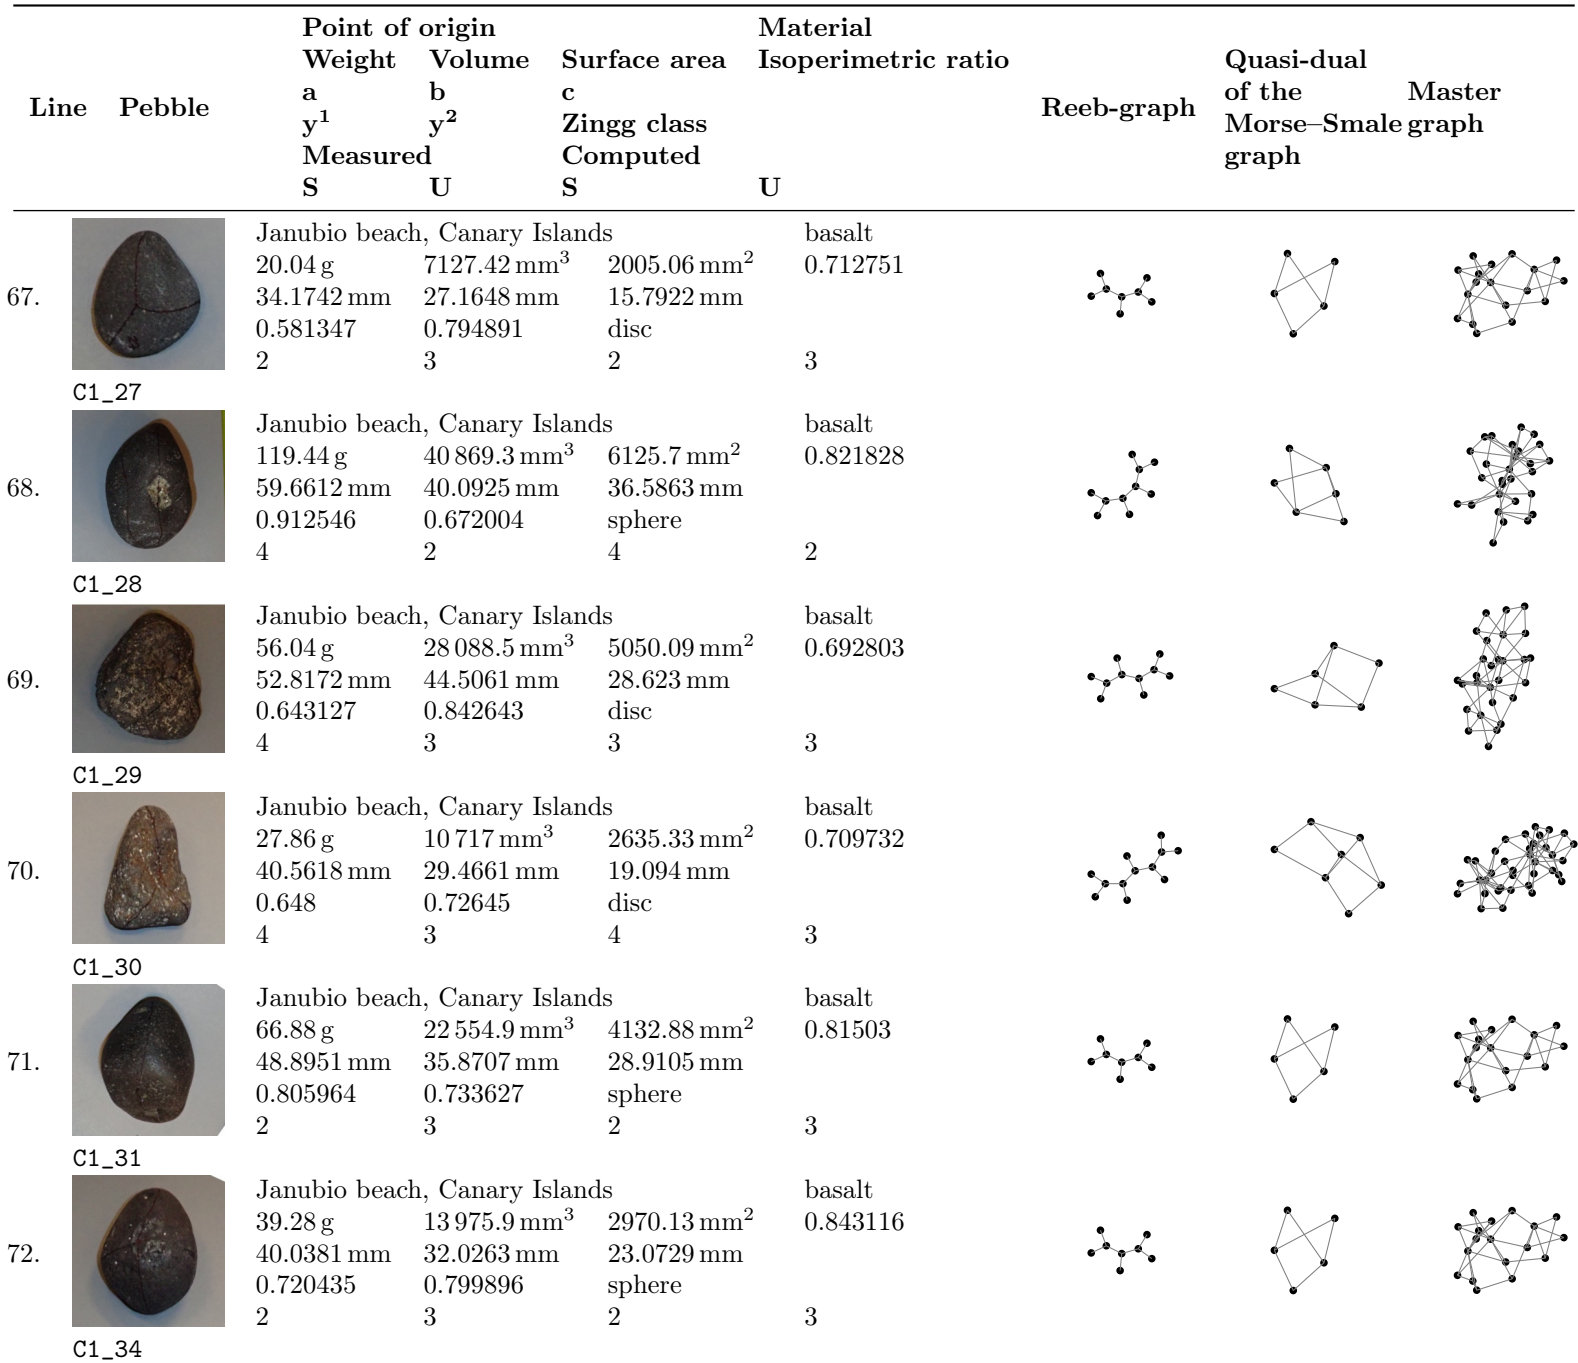   | 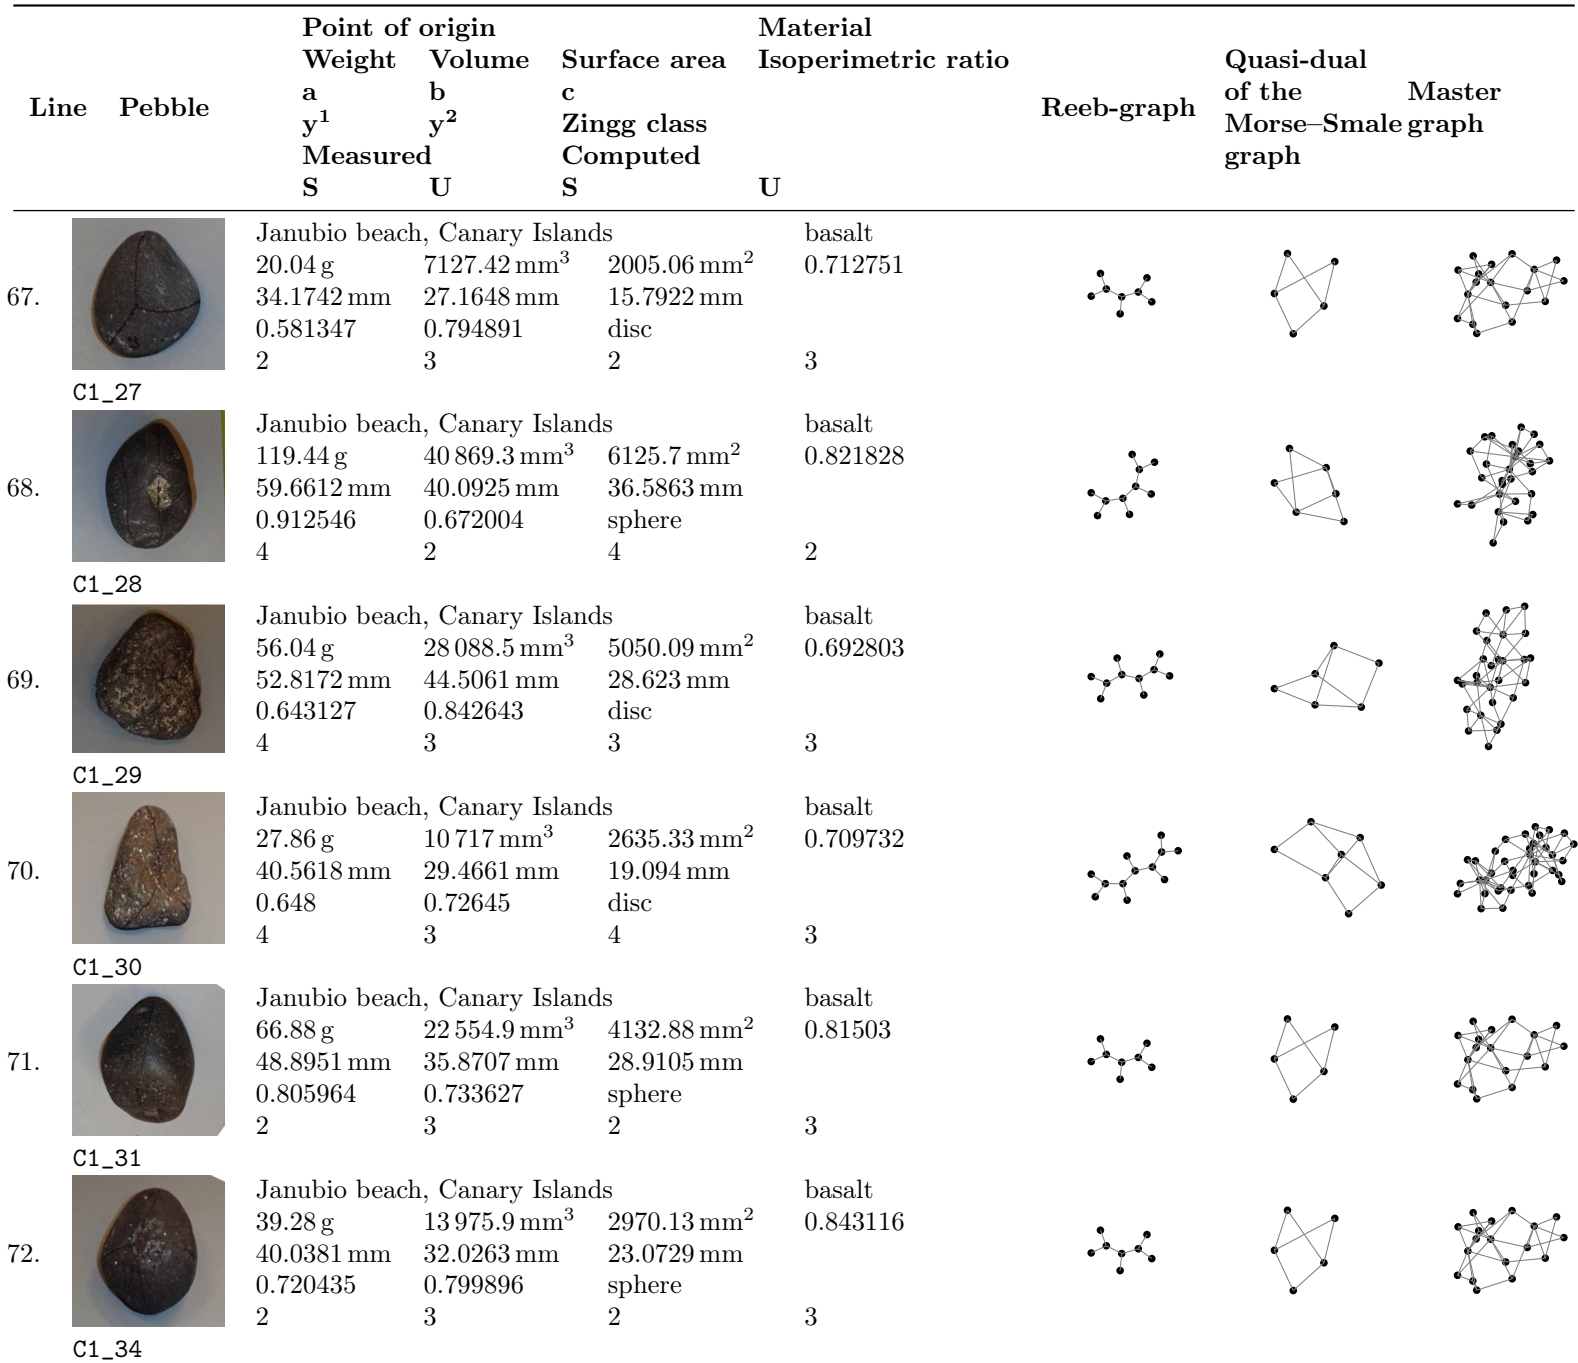   |
|      |                                                                                     | 20.04 g                       | 7127.42 mm <sup>3</sup>  | 2005.06 mm <sup>2</sup> |          |                     |                                                                                       |                                                                                       |                                                                                       |
|      |                                                                                     | 34.1742 mm                    | 27.1648 mm               | 15.7922 mm              |          |                     |                                                                                       |                                                                                       |                                                                                       |
|      |                                                                                     | 0.581347                      | 0.794891                 | disc                    |          |                     |                                                                                       |                                                                                       |                                                                                       |
|      |                                                                                     | 2                             | 3                        | 2                       |          |                     |                                                                                       |                                                                                       |                                                                                       |
|      | C1_27                                                                               |                               |                          |                         |          |                     |                                                                                       |                                                                                       |                                                                                       |
| 68.  | 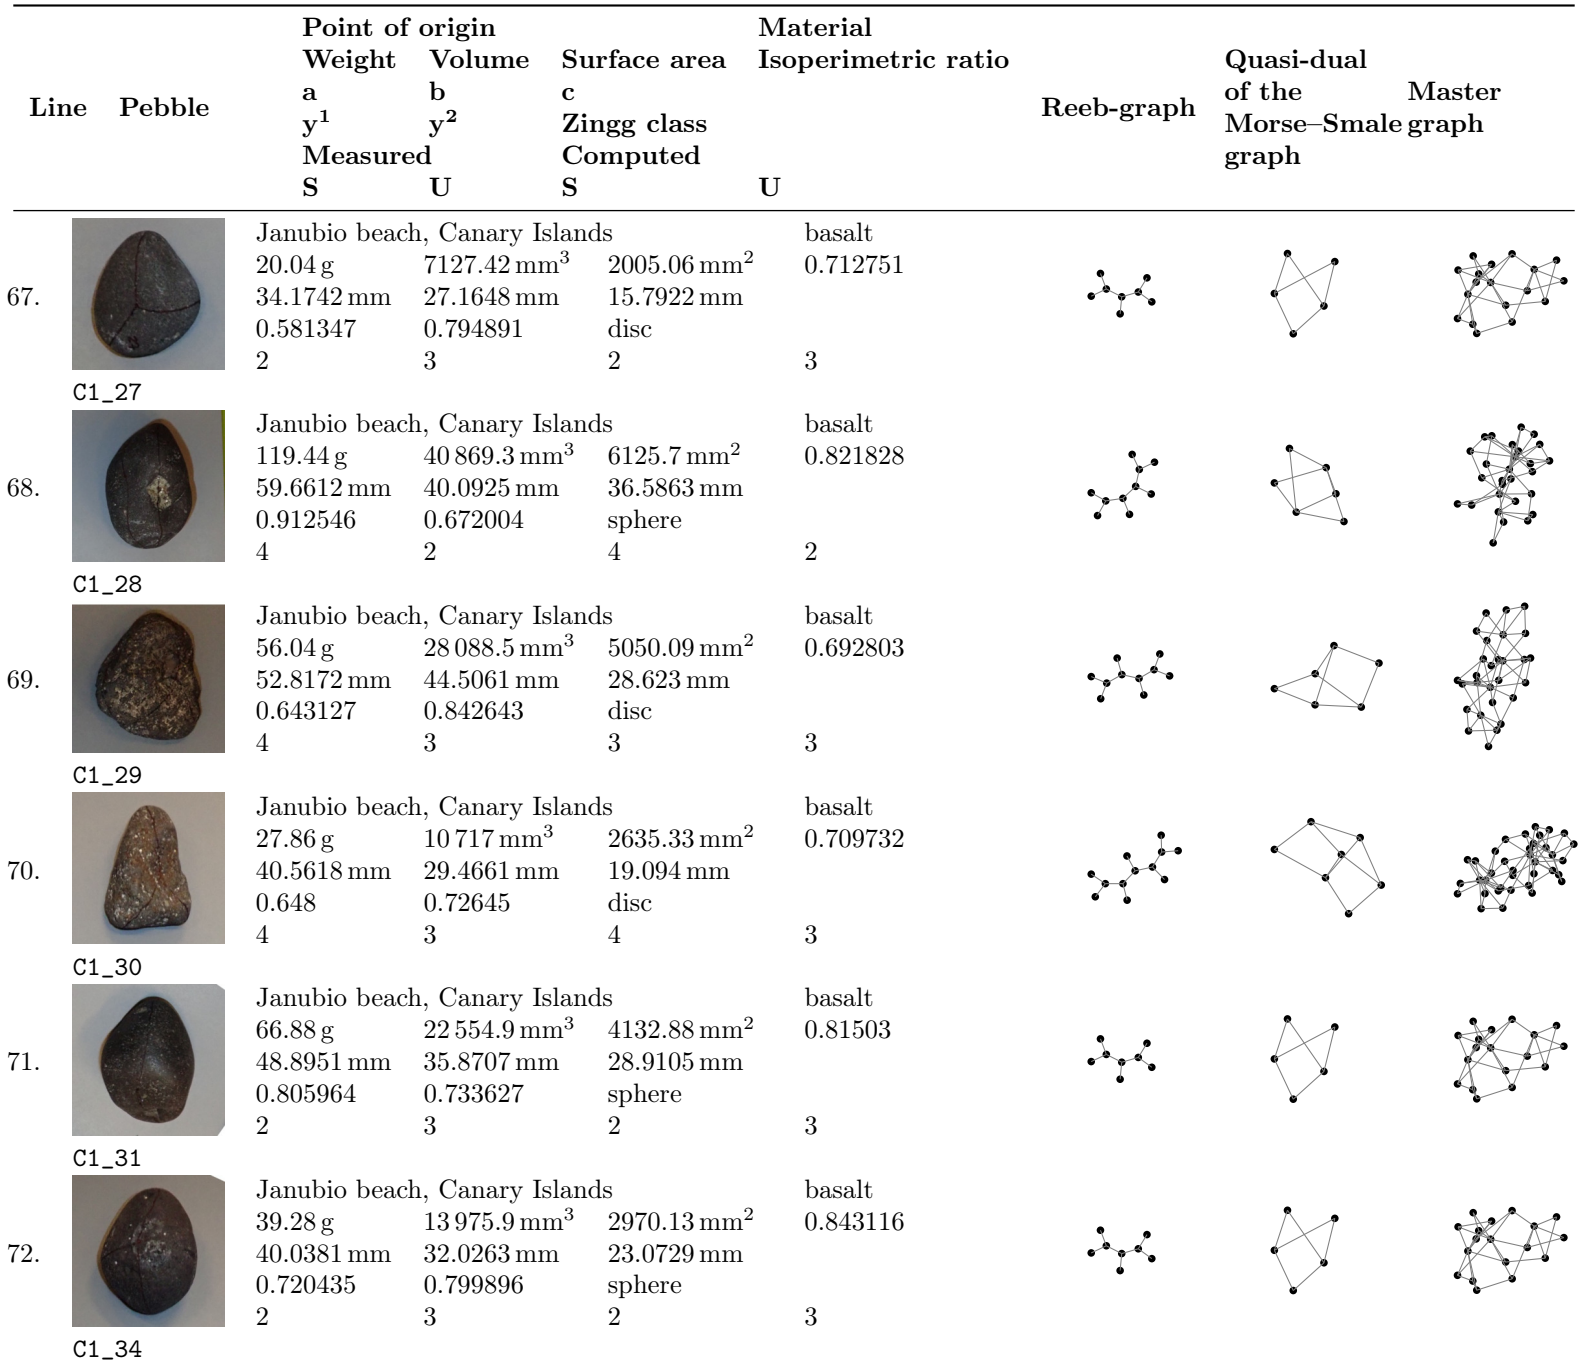   | Janubio beach, Canary Islands |                          |                         | basalt   | 0.821828            | 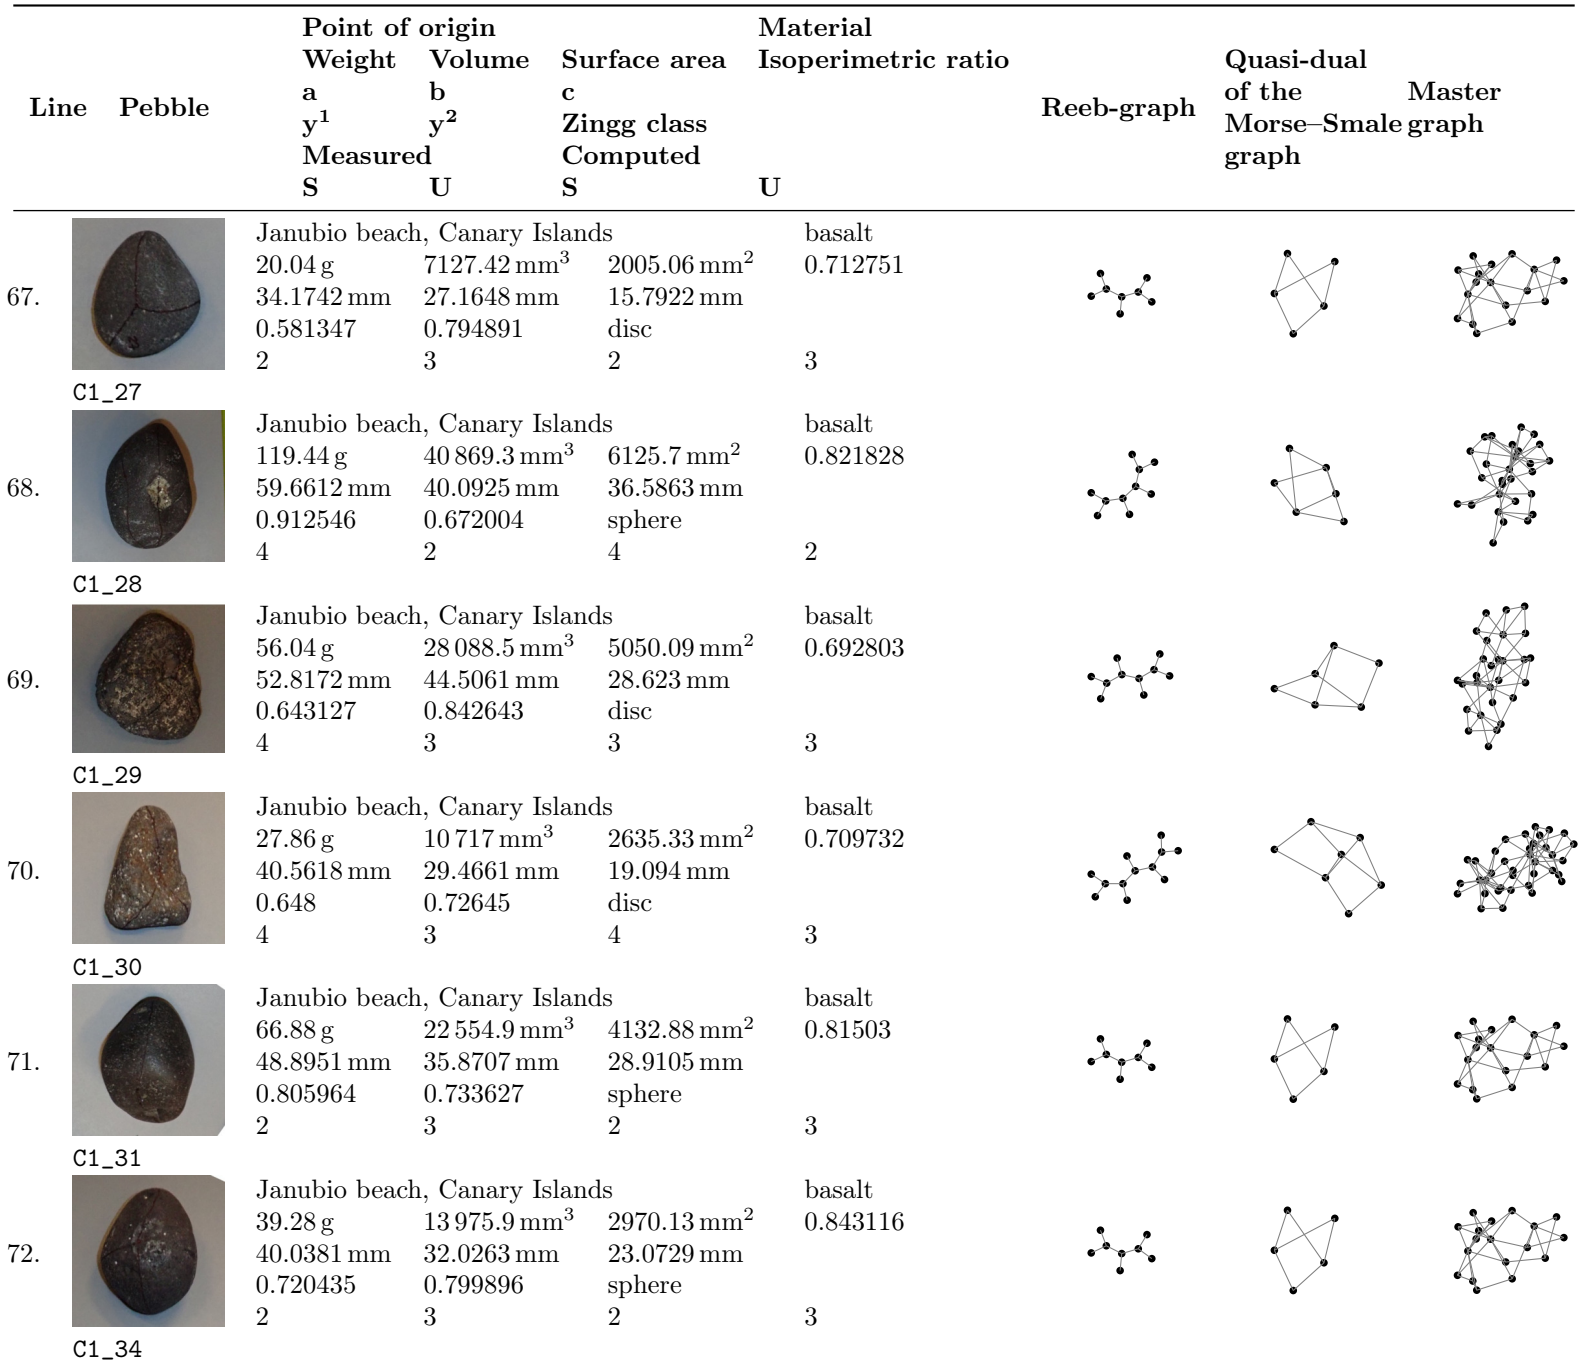   | 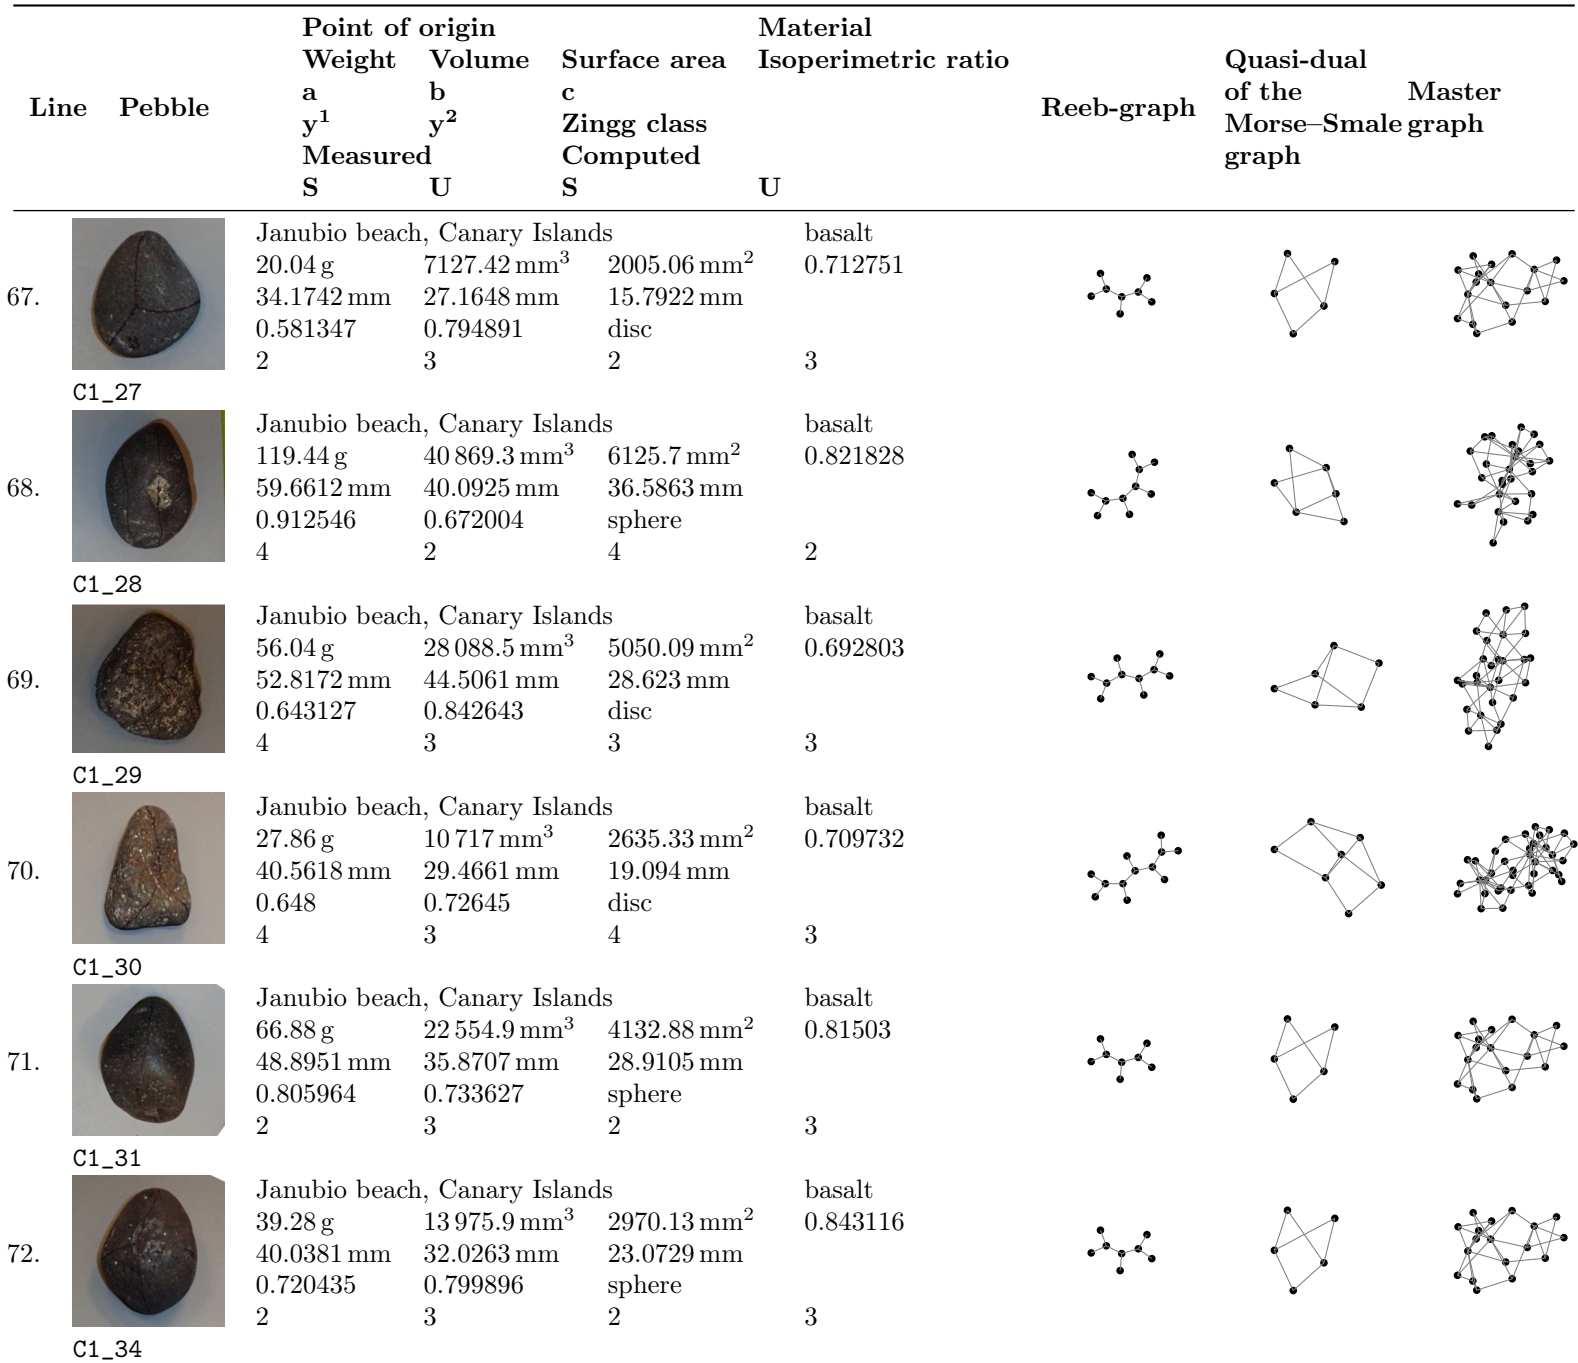   | 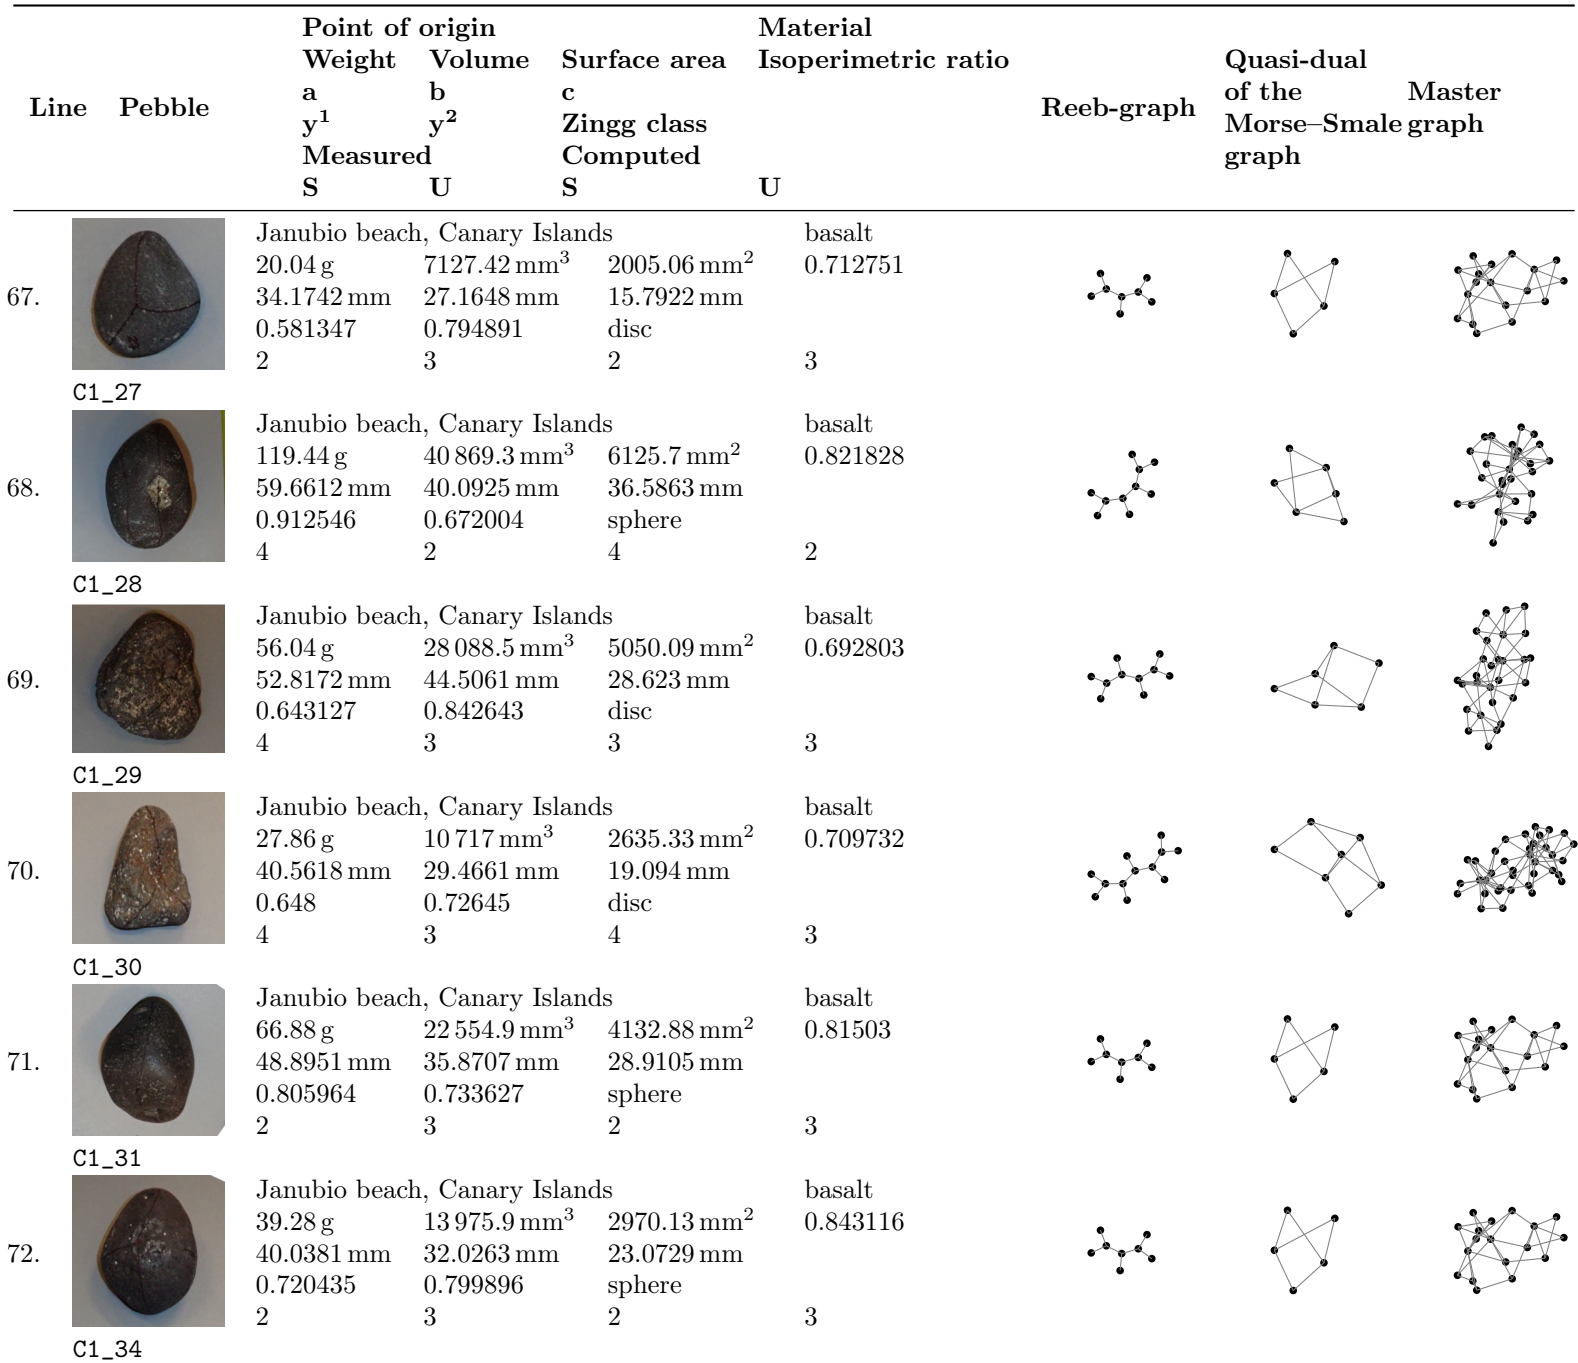   |
|      |                                                                                     | 119.44 g                      | 40 869.3 mm <sup>3</sup> | 6125.7 mm <sup>2</sup>  |          |                     |                                                                                       |                                                                                       |                                                                                       |
|      |                                                                                     | 59.6612 mm                    | 40.0925 mm               | 36.5863 mm              |          |                     |                                                                                       |                                                                                       |                                                                                       |
|      |                                                                                     | 0.912546                      | 0.672004                 | sphere                  |          |                     |                                                                                       |                                                                                       |                                                                                       |
|      |                                                                                     | 4                             | 2                        | 4                       |          |                     |                                                                                       |                                                                                       |                                                                                       |
|      | C1_28                                                                               |                               |                          |                         |          |                     |                                                                                       |                                                                                       |                                                                                       |
| 69.  | 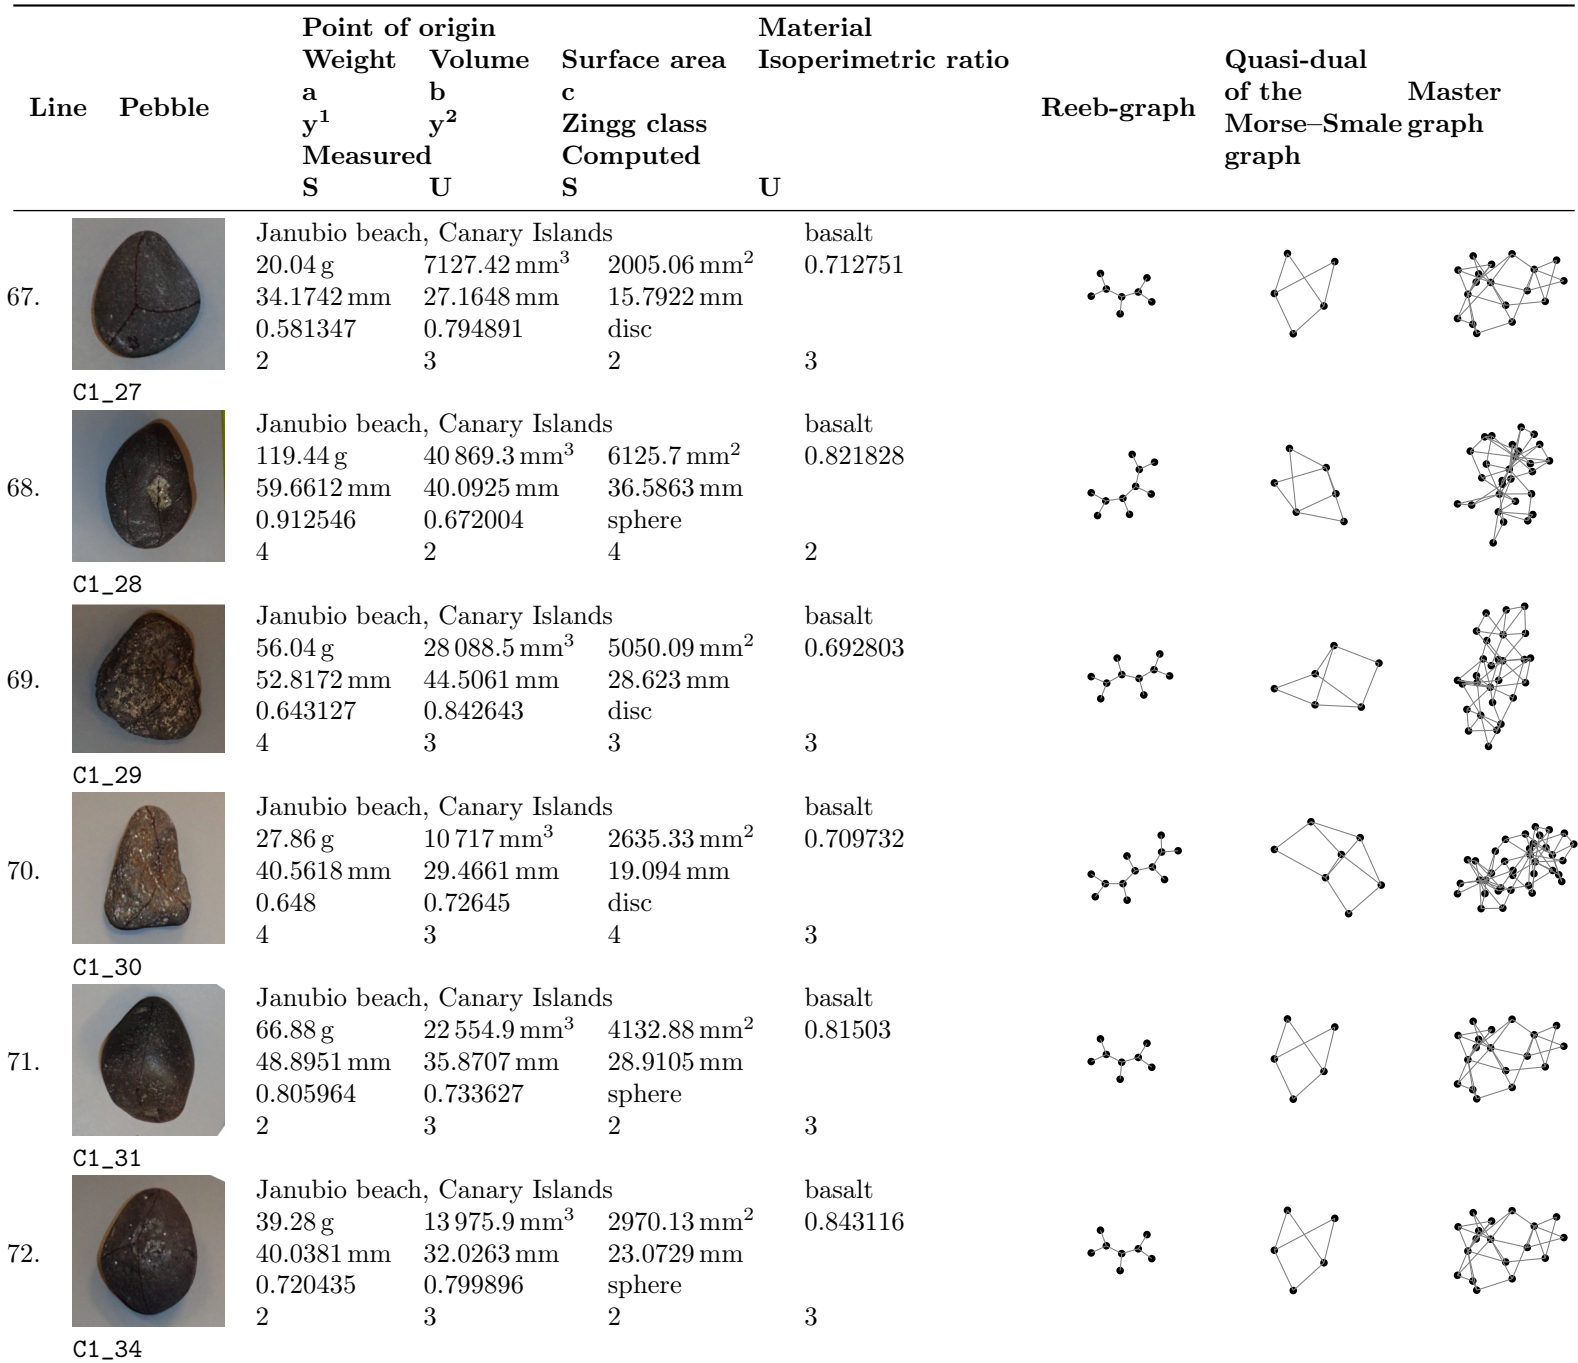   | Janubio beach, Canary Islands |                          |                         | basalt   | 0.692803            | 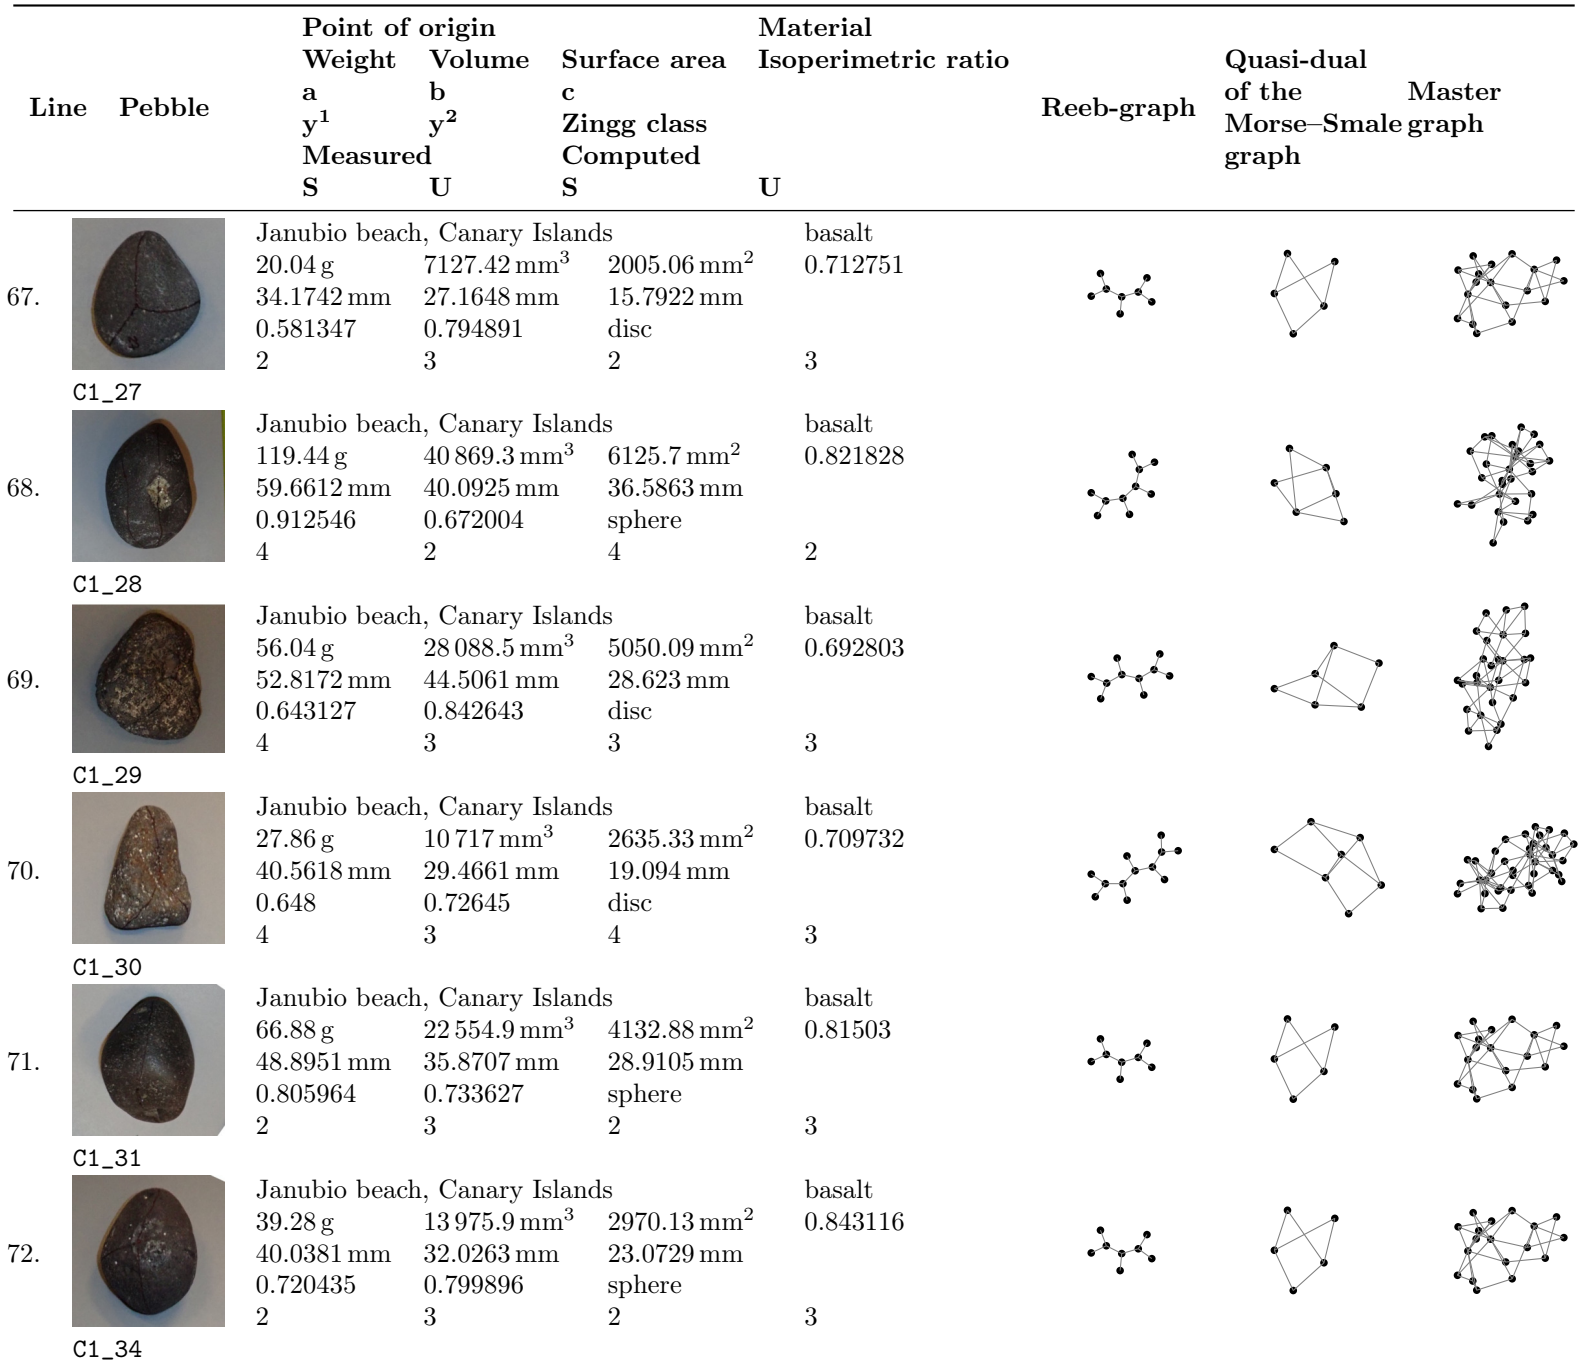   | 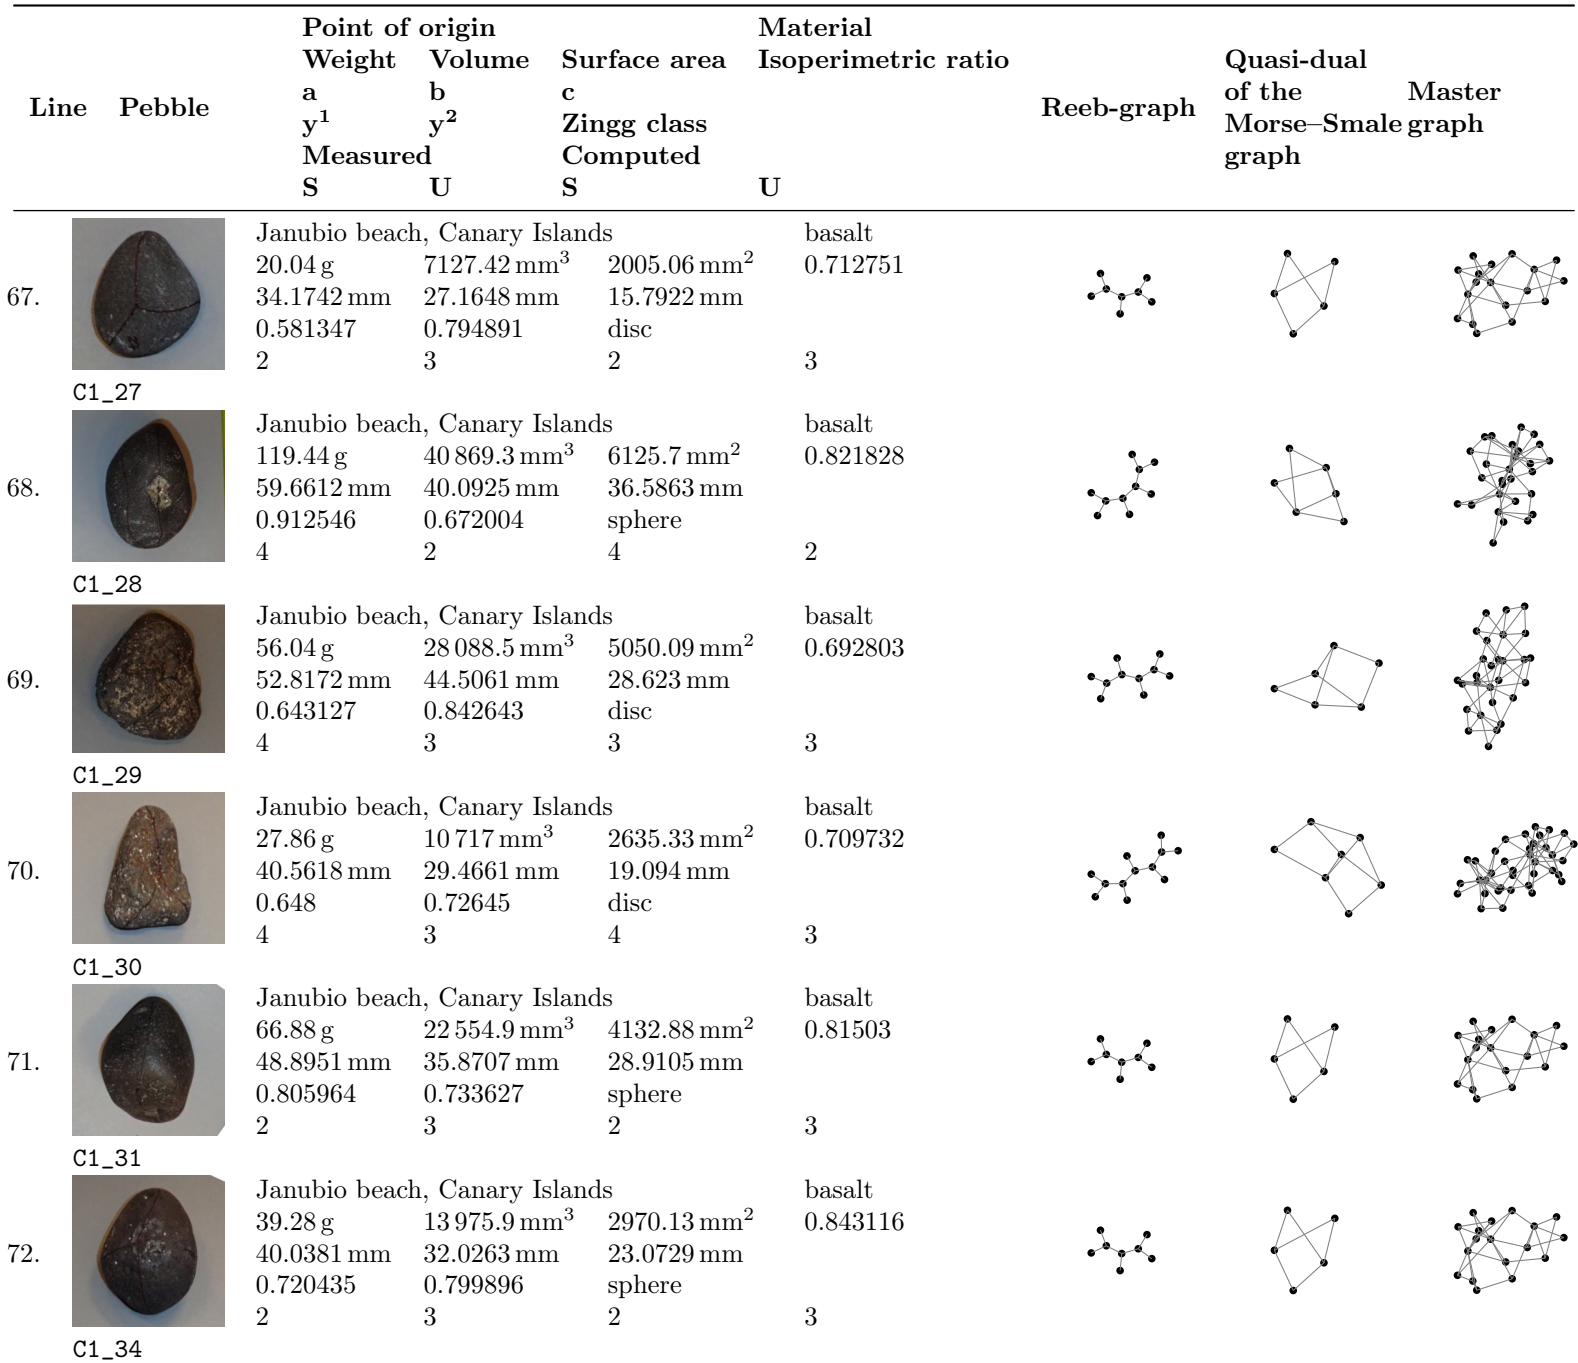   | 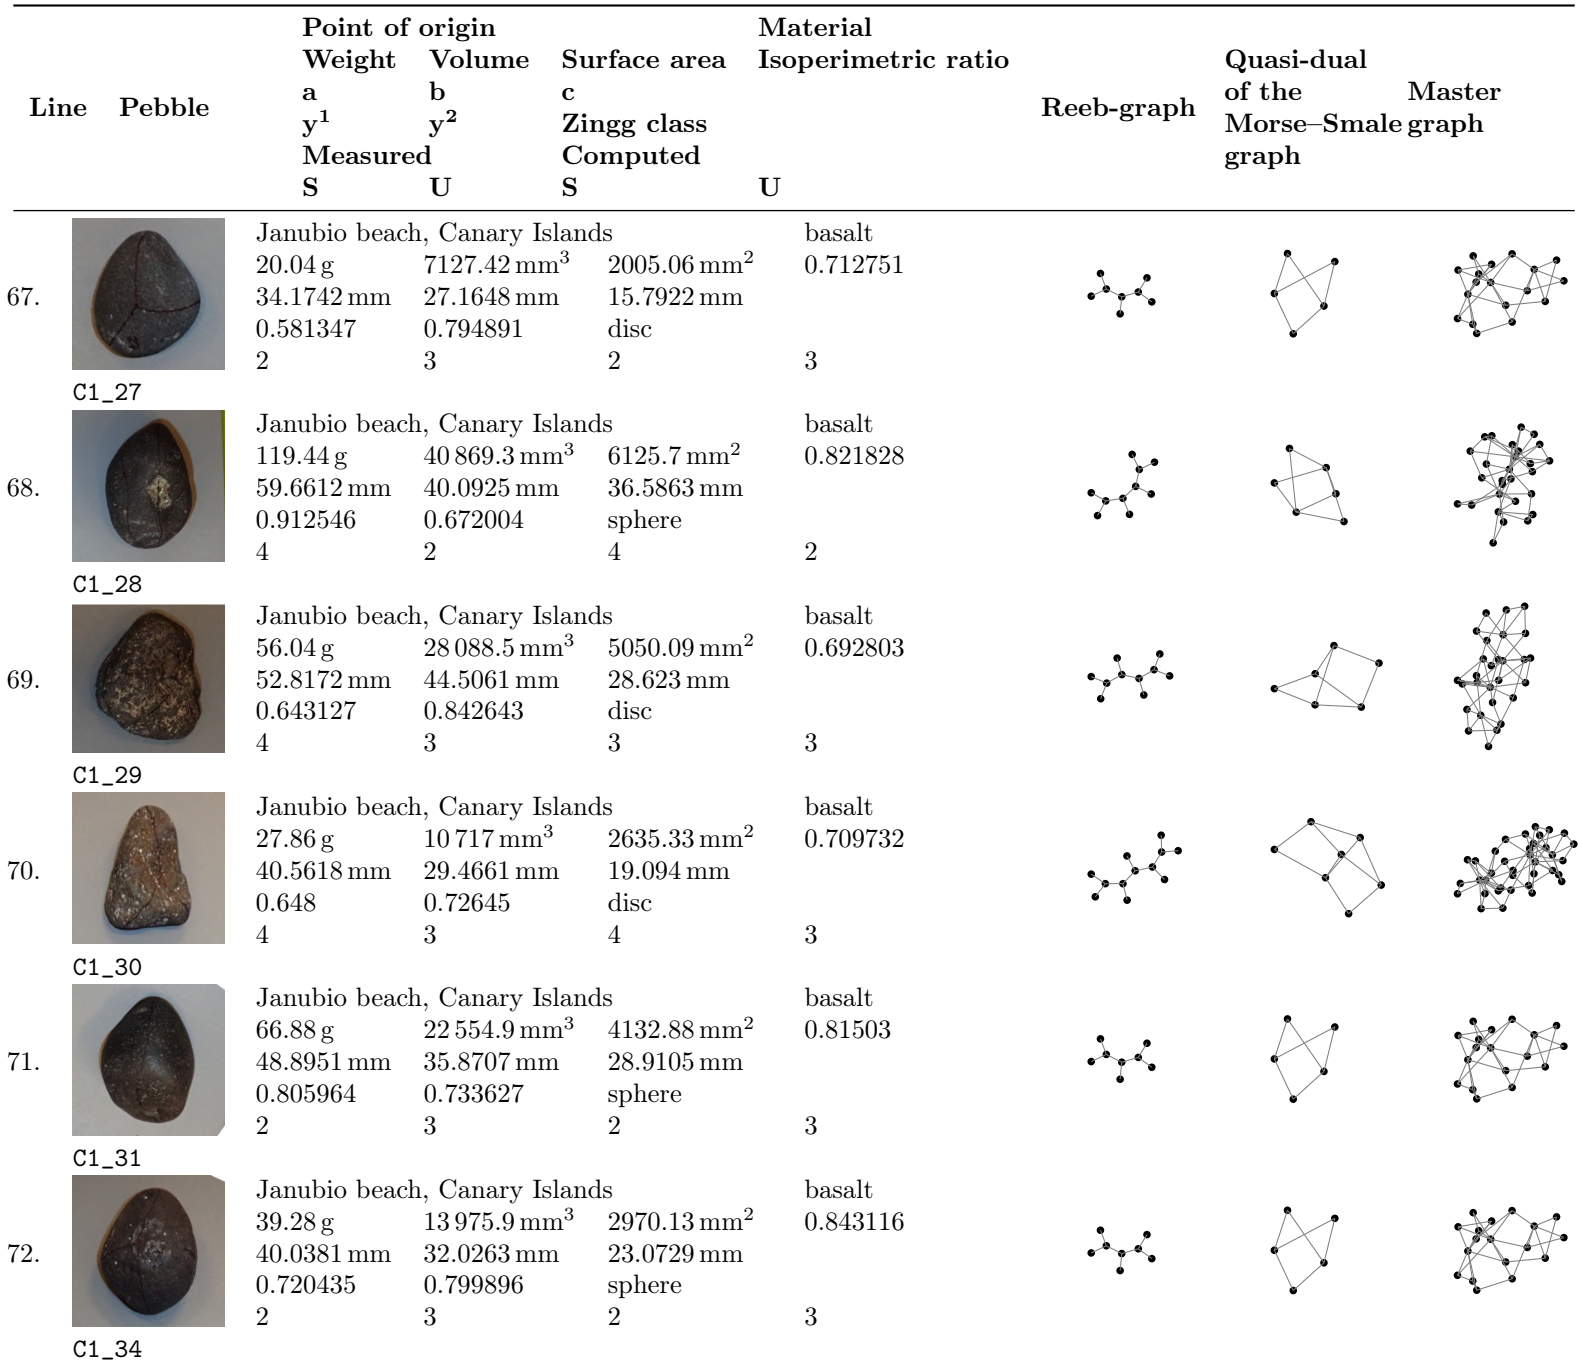   |
|      |                                                                                     | 56.04 g                       | 28 088.5 mm <sup>3</sup> | 5050.09 mm <sup>2</sup> |          |                     |                                                                                       |                                                                                       |                                                                                       |
|      |                                                                                     | 52.8172 mm                    | 44.5061 mm               | 28.623 mm               |          |                     |                                                                                       |                                                                                       |                                                                                       |
|      |                                                                                     | 0.643127                      | 0.842643                 | disc                    |          |                     |                                                                                       |                                                                                       |                                                                                       |
|      |                                                                                     | 4                             | 3                        | 3                       |          |                     |                                                                                       |                                                                                       |                                                                                       |
|      | C1_29                                                                               |                               |                          |                         |          |                     |                                                                                       |                                                                                       |                                                                                       |
| 70.  | 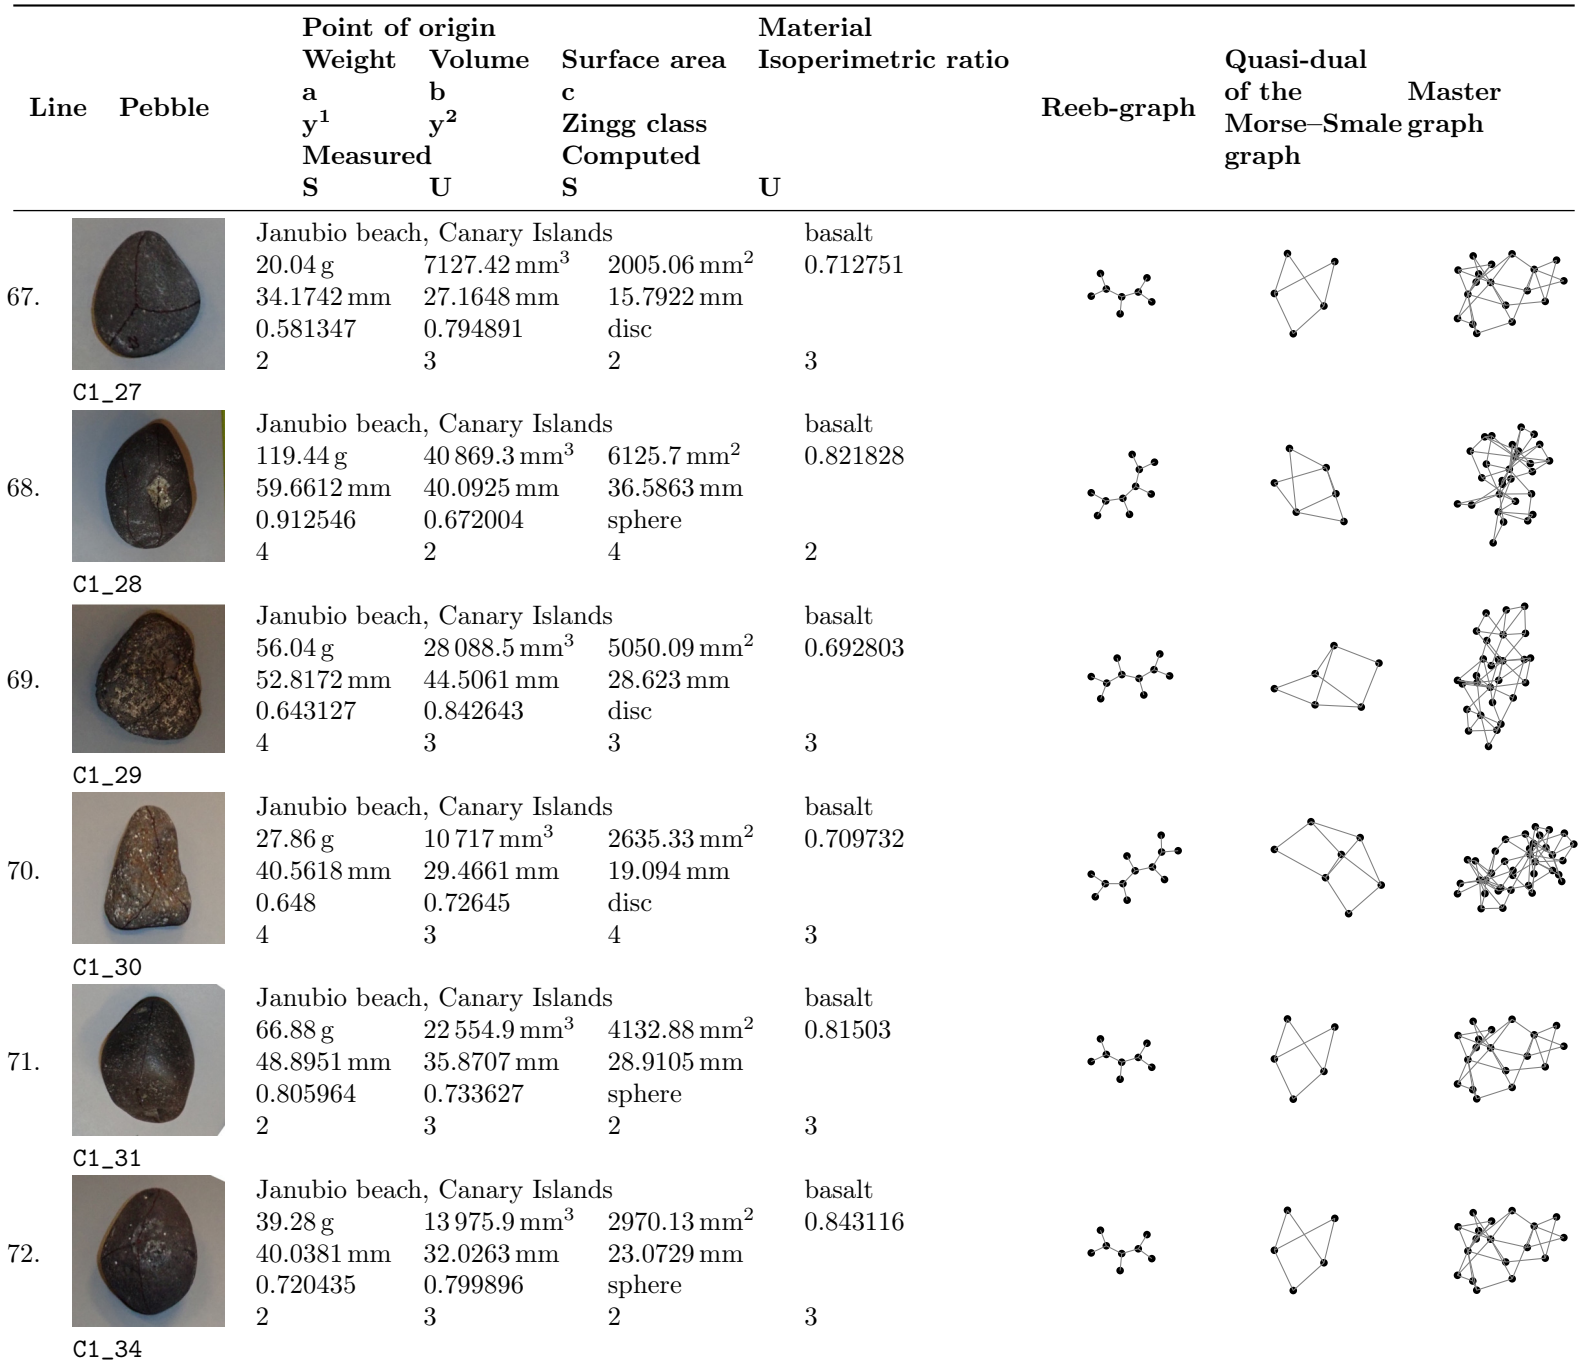  | Janubio beach, Canary Islands |                          |                         | basalt   | 0.709732            | 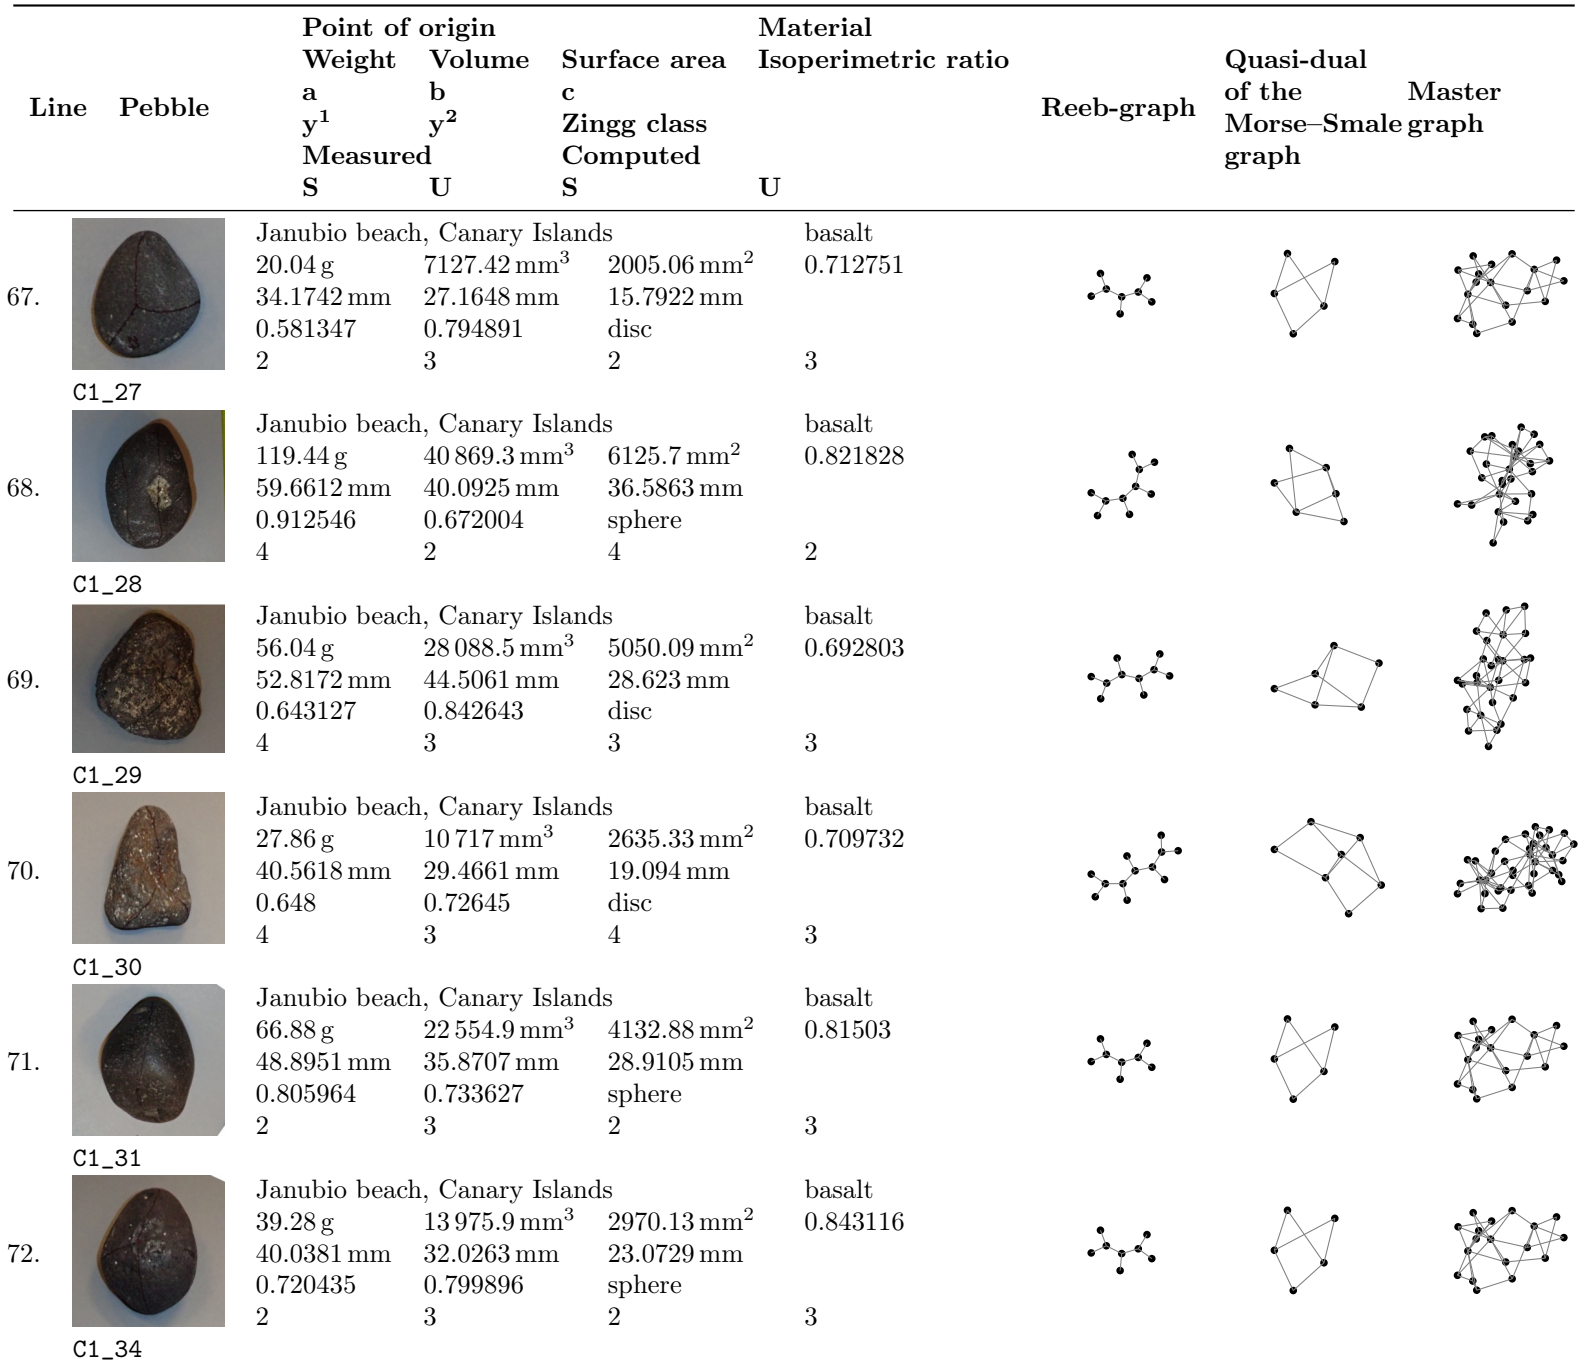  | 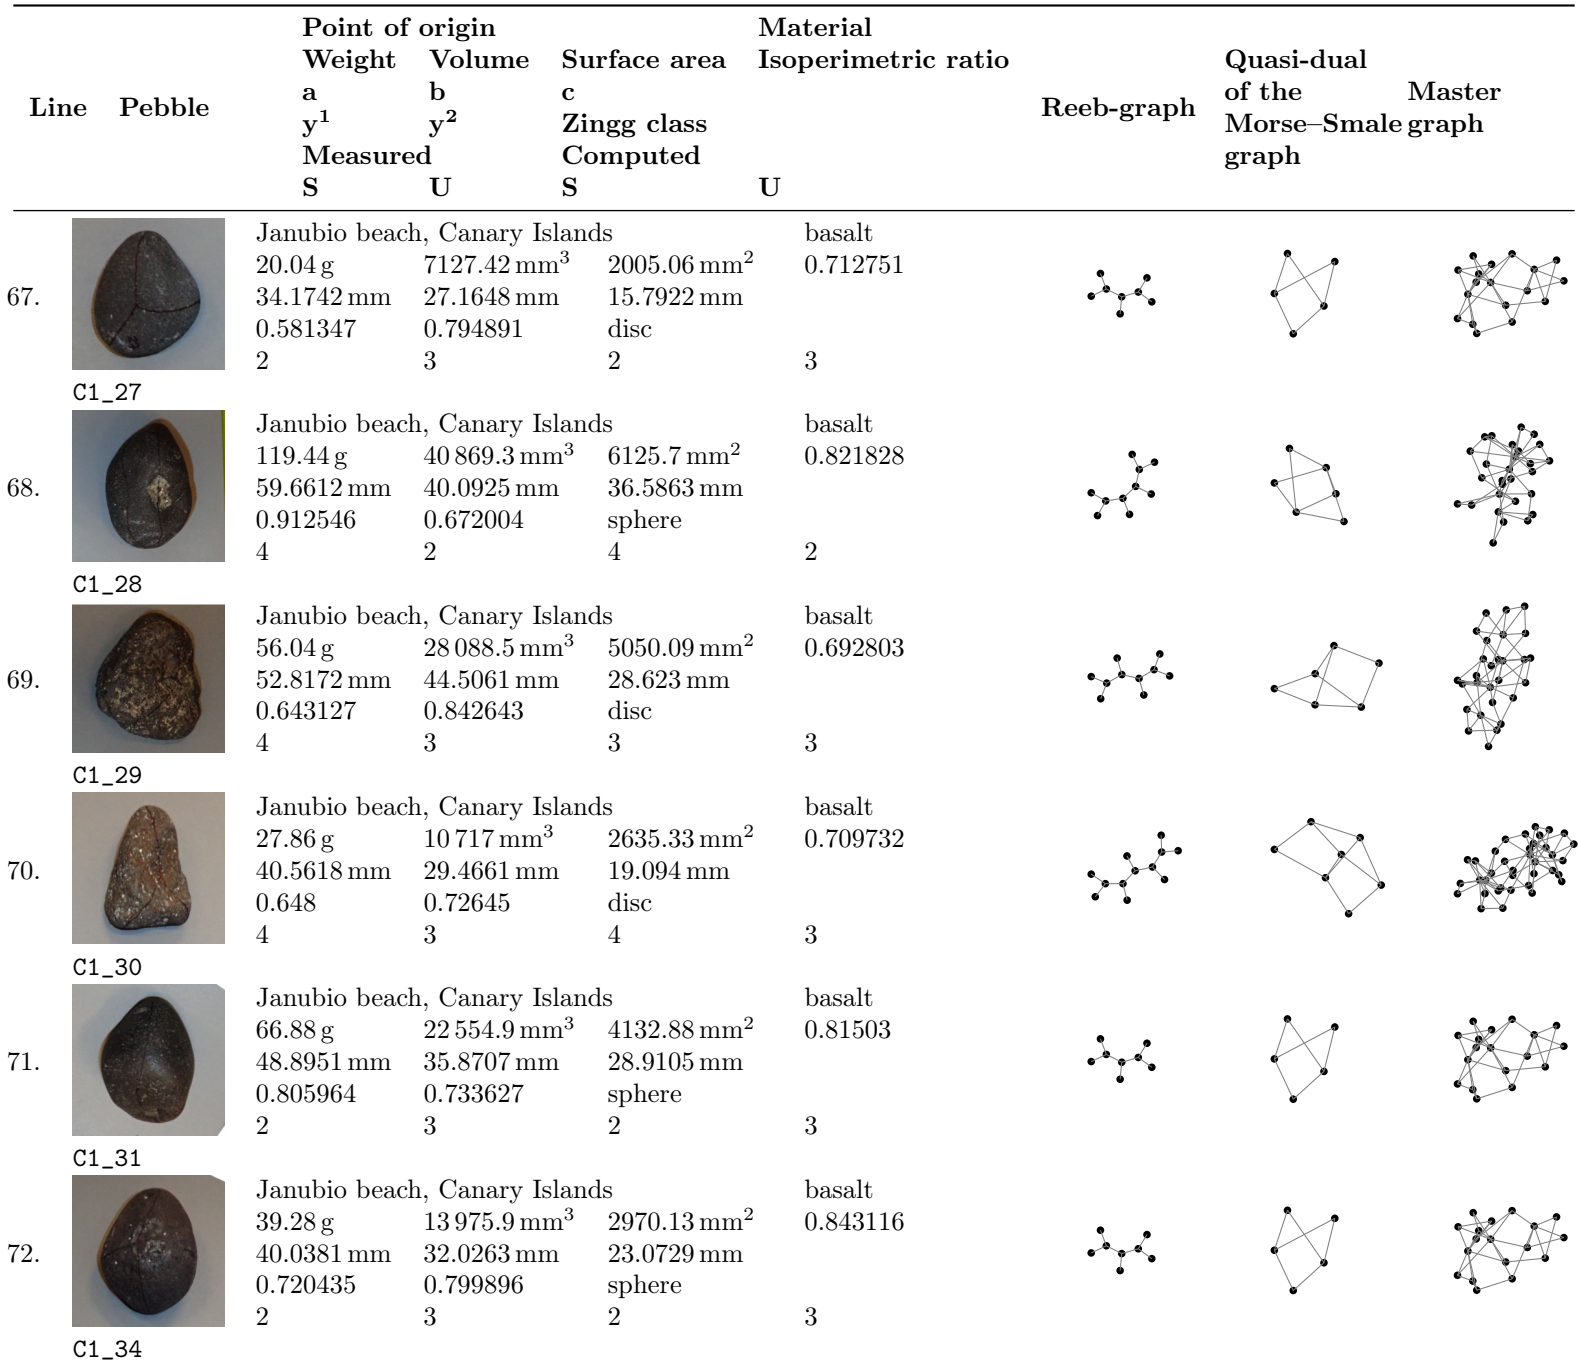  | 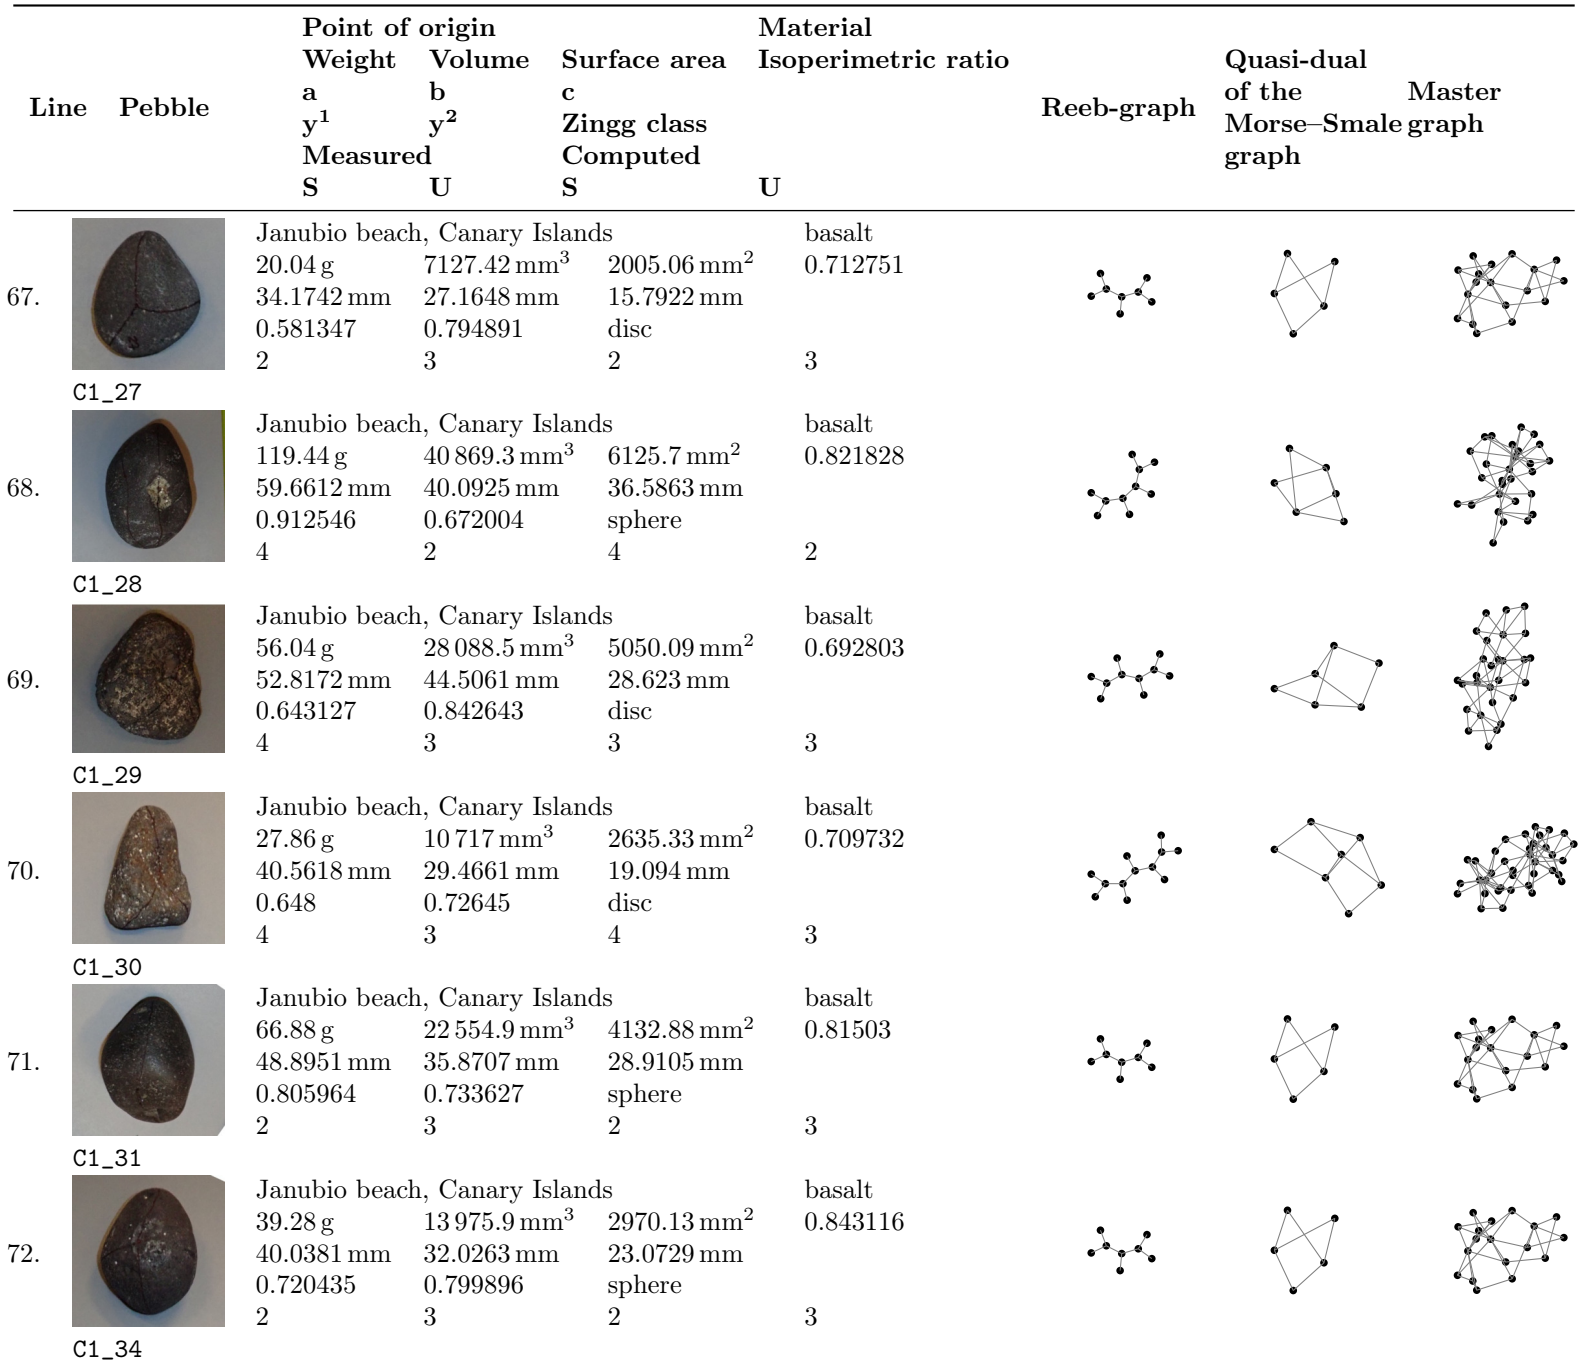  |
|      |                                                                                     | 27.86 g                       | 10 717 mm <sup>3</sup>   | 2635.33 mm <sup>2</sup> |          |                     |                                                                                       |                                                                                       |                                                                                       |
|      |                                                                                     | 40.5618 mm                    | 29.4661 mm               | 19.094 mm               |          |                     |                                                                                       |                                                                                       |                                                                                       |
|      |                                                                                     | 0.648                         | 0.72645                  | disc                    |          |                     |                                                                                       |                                                                                       |                                                                                       |
|      |                                                                                     | 4                             | 3                        | 4                       |          |                     |                                                                                       |                                                                                       |                                                                                       |
|      | C1_30                                                                               |                               |                          |                         |          |                     |                                                                                       |                                                                                       |                                                                                       |
| 71.  | 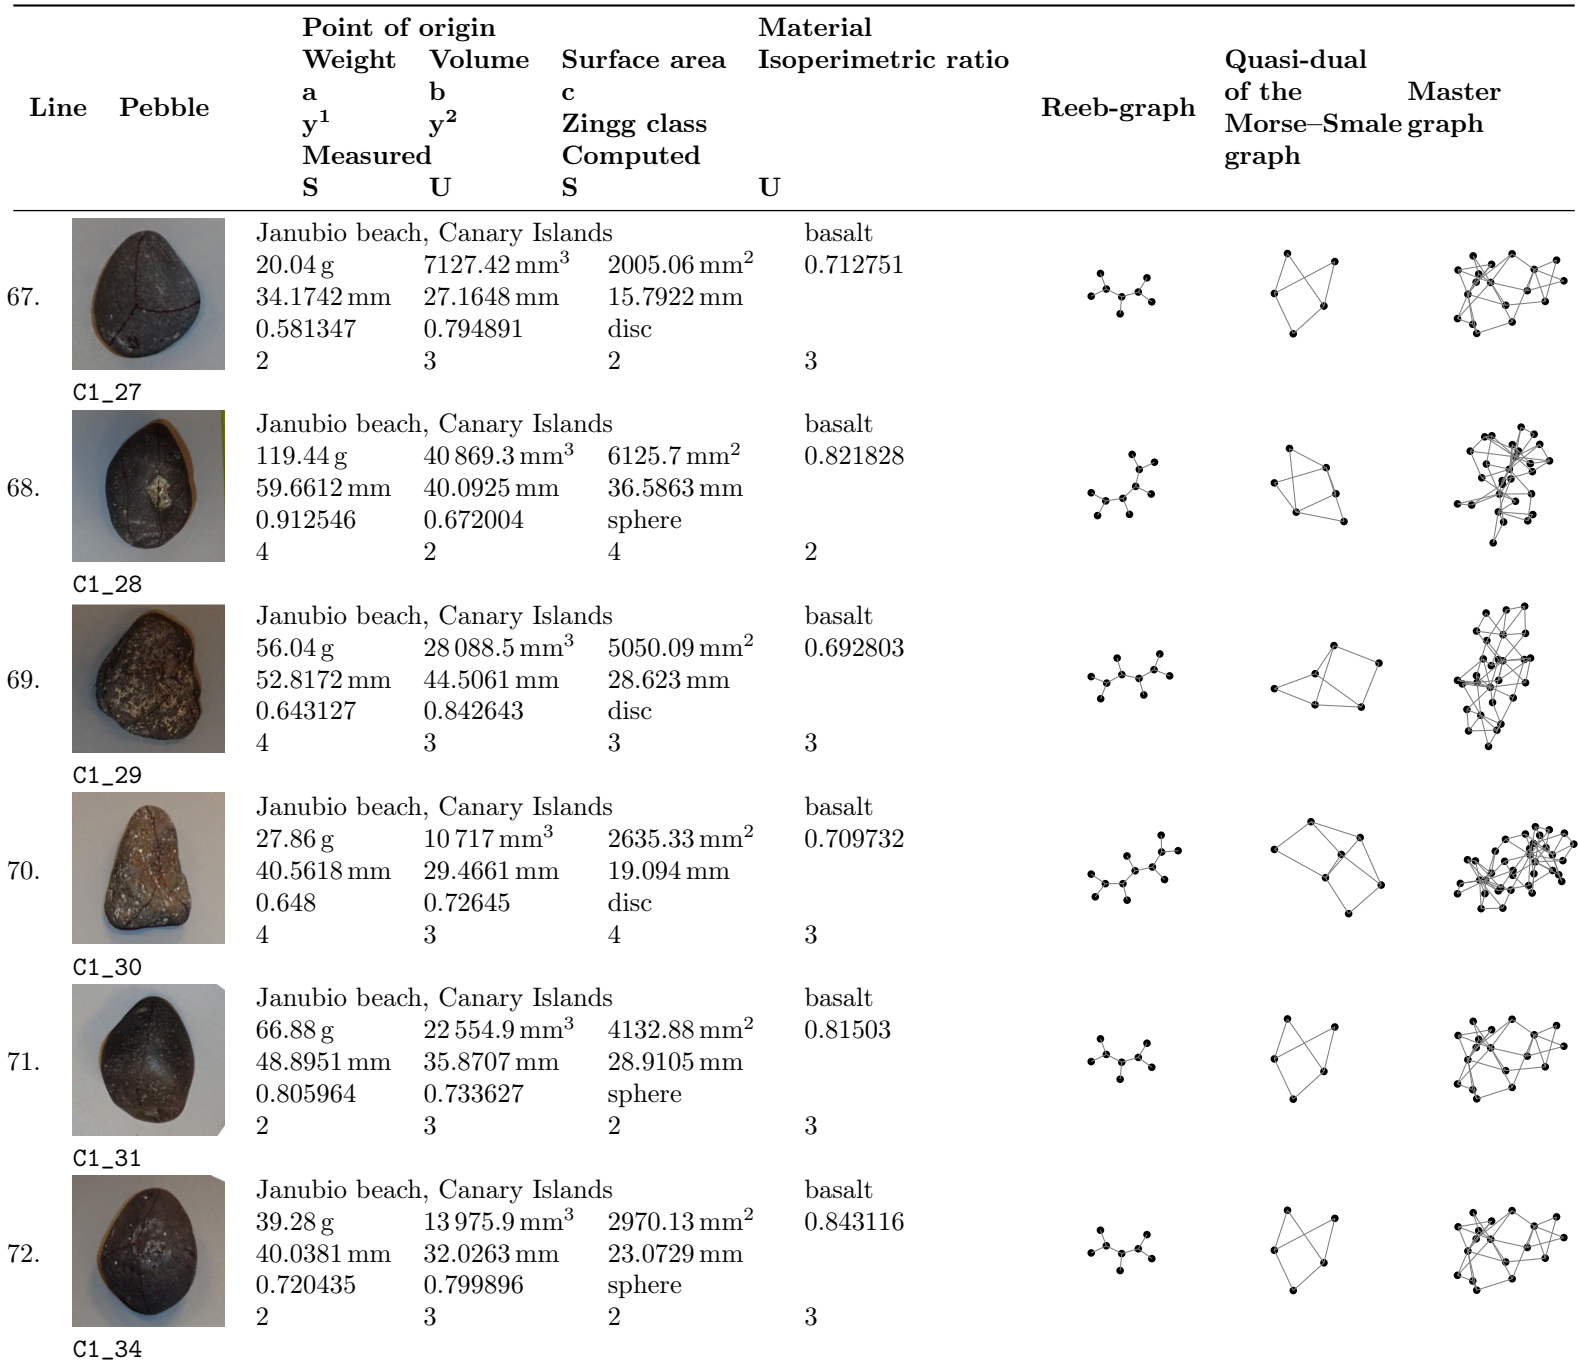 | Janubio beach, Canary Islands |                          |                         | basalt   | 0.81503             | 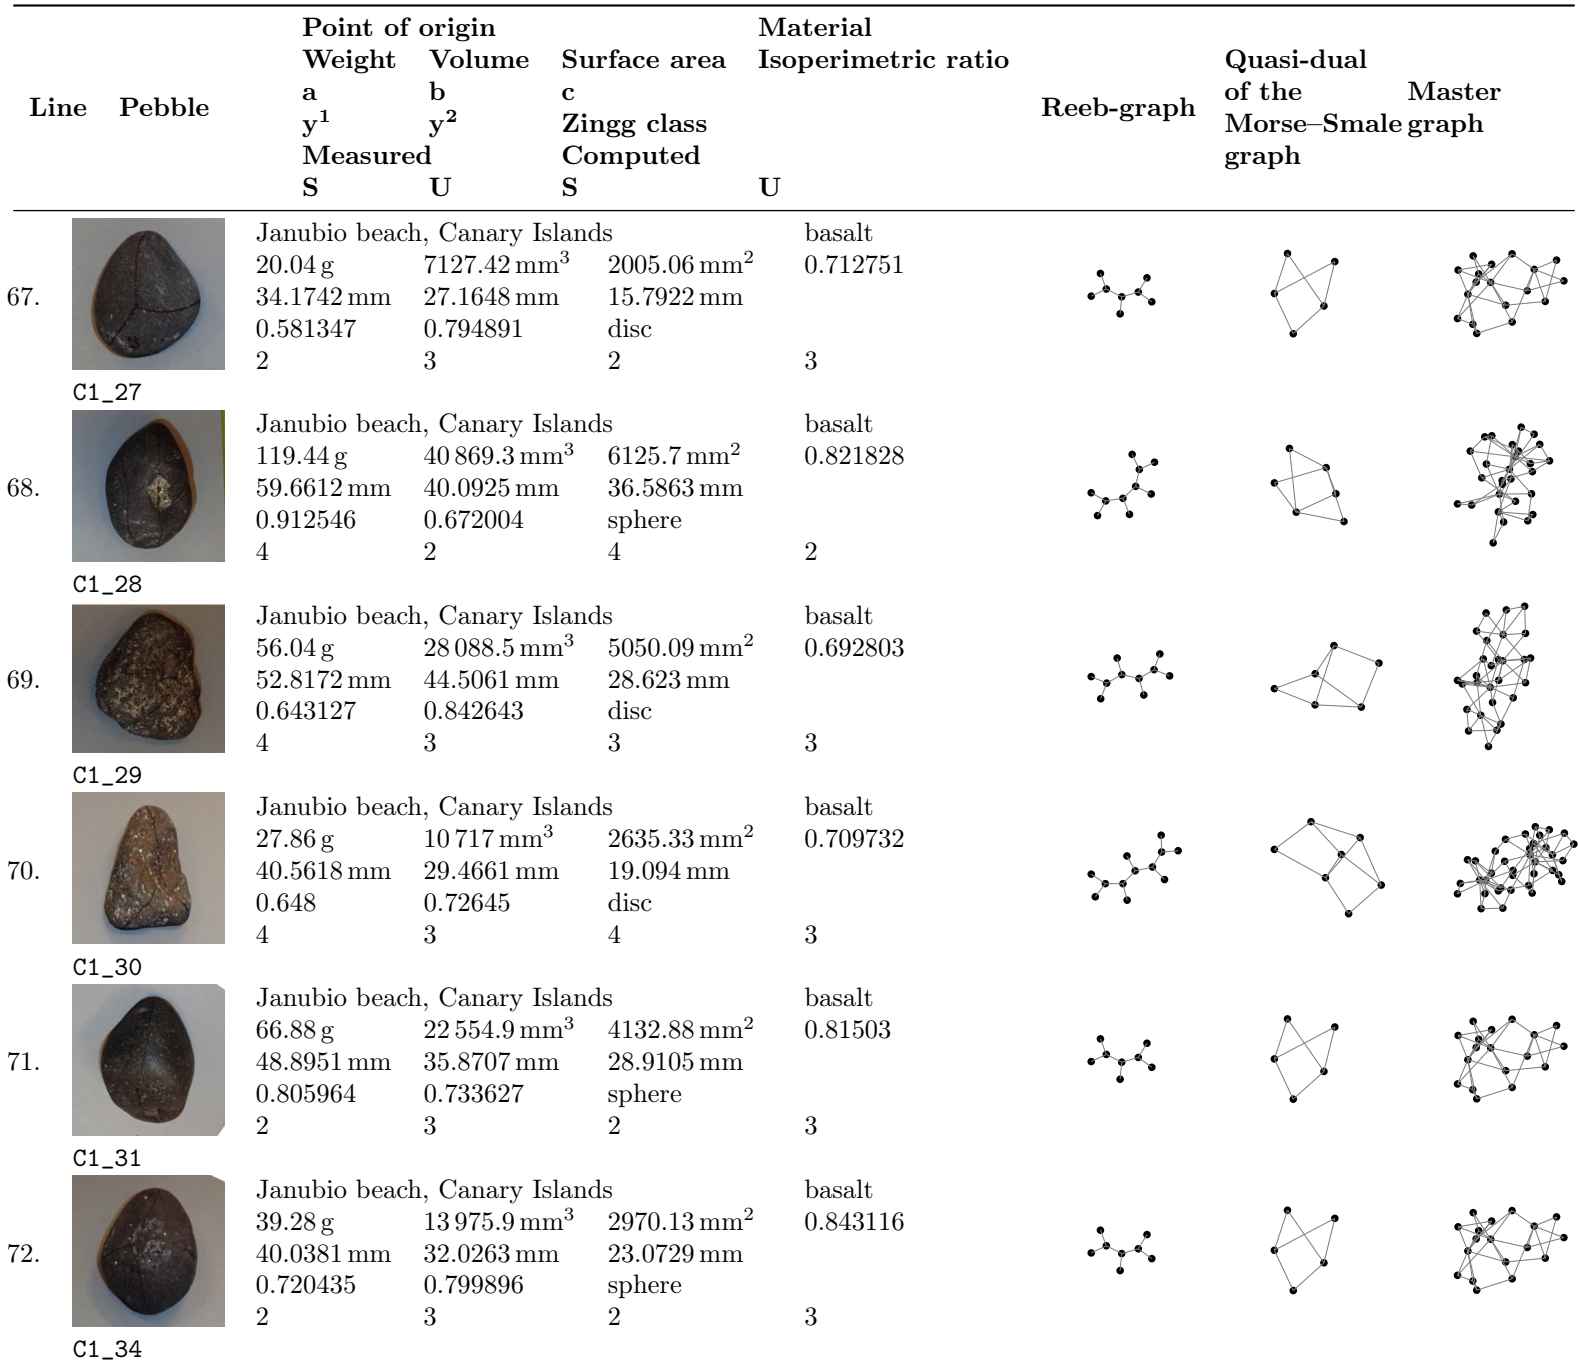 | 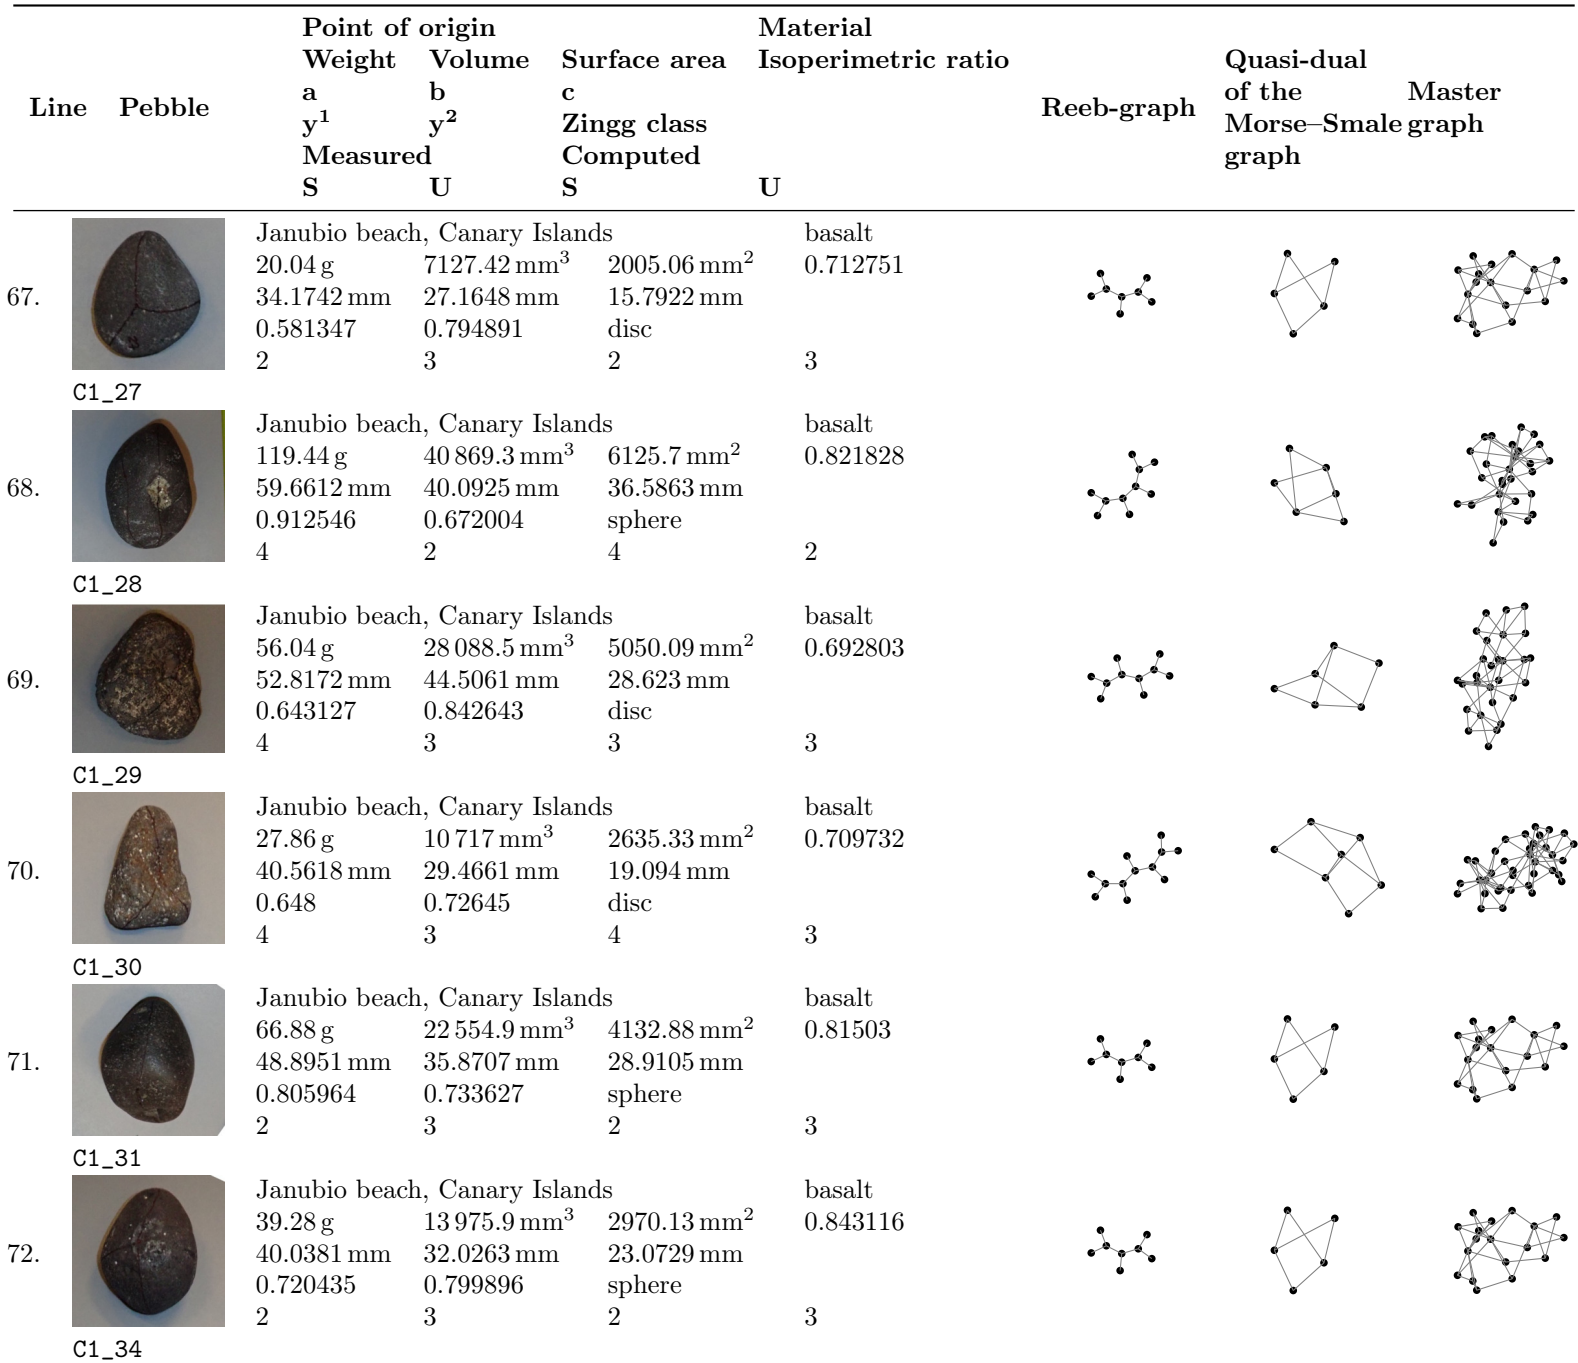 | 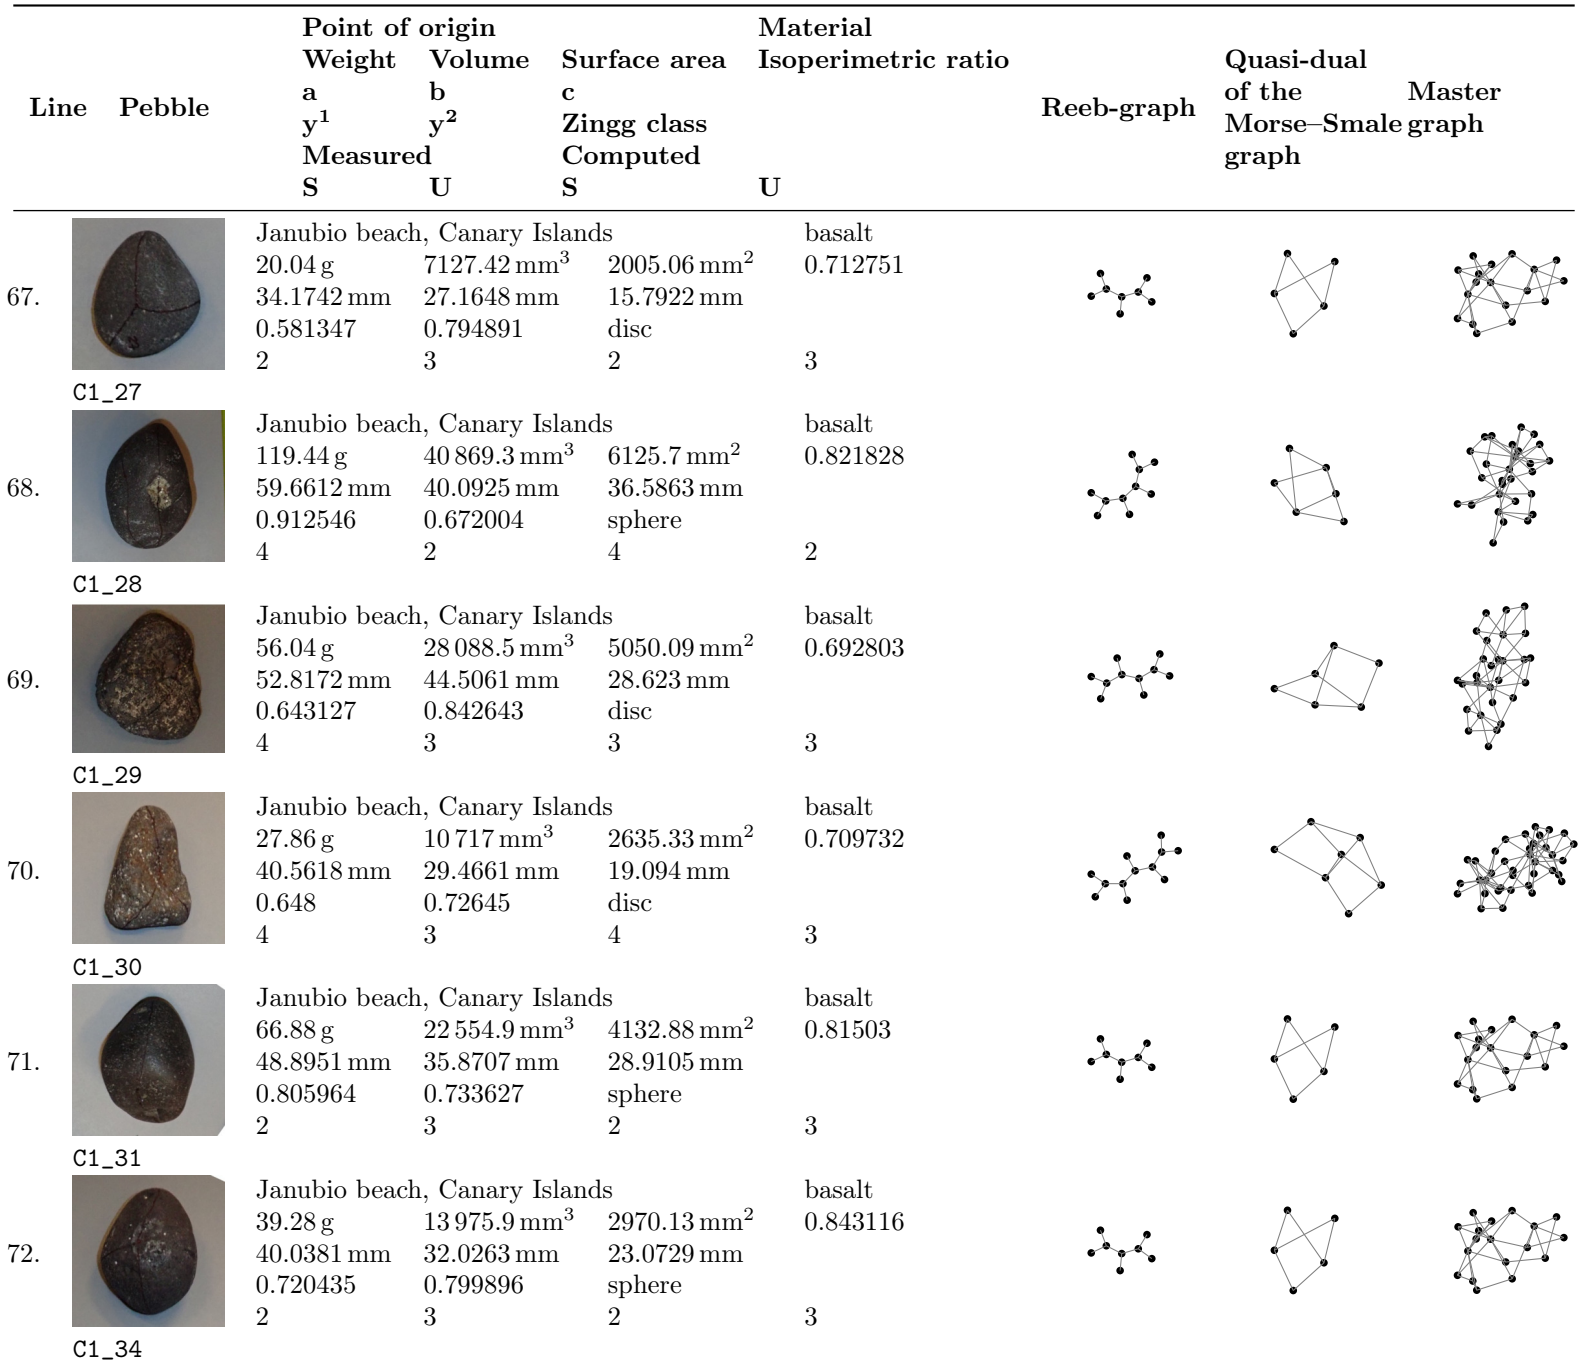 |
|      |                                                                                     | 66.88 g                       | 22 554.9 mm <sup>3</sup> | 4132.88 mm <sup>2</sup> |          |                     |                                                                                       |                                                                                       |                                                                                       |
|      |                                                                                     | 48.8951 mm                    | 35.8707 mm               | 28.9105 mm              |          |                     |                                                                                       |                                                                                       |                                                                                       |
|      |                                                                                     | 0.805964                      | 0.733627                 | sphere                  |          |                     |                                                                                       |                                                                                       |                                                                                       |
|      |                                                                                     | 2                             | 3                        | 2                       |          |                     |                                                                                       |                                                                                       |                                                                                       |
|      | C1_31                                                                               |                               |                          |                         |          |                     |                                                                                       |                                                                                       |                                                                                       |
| 72.  | 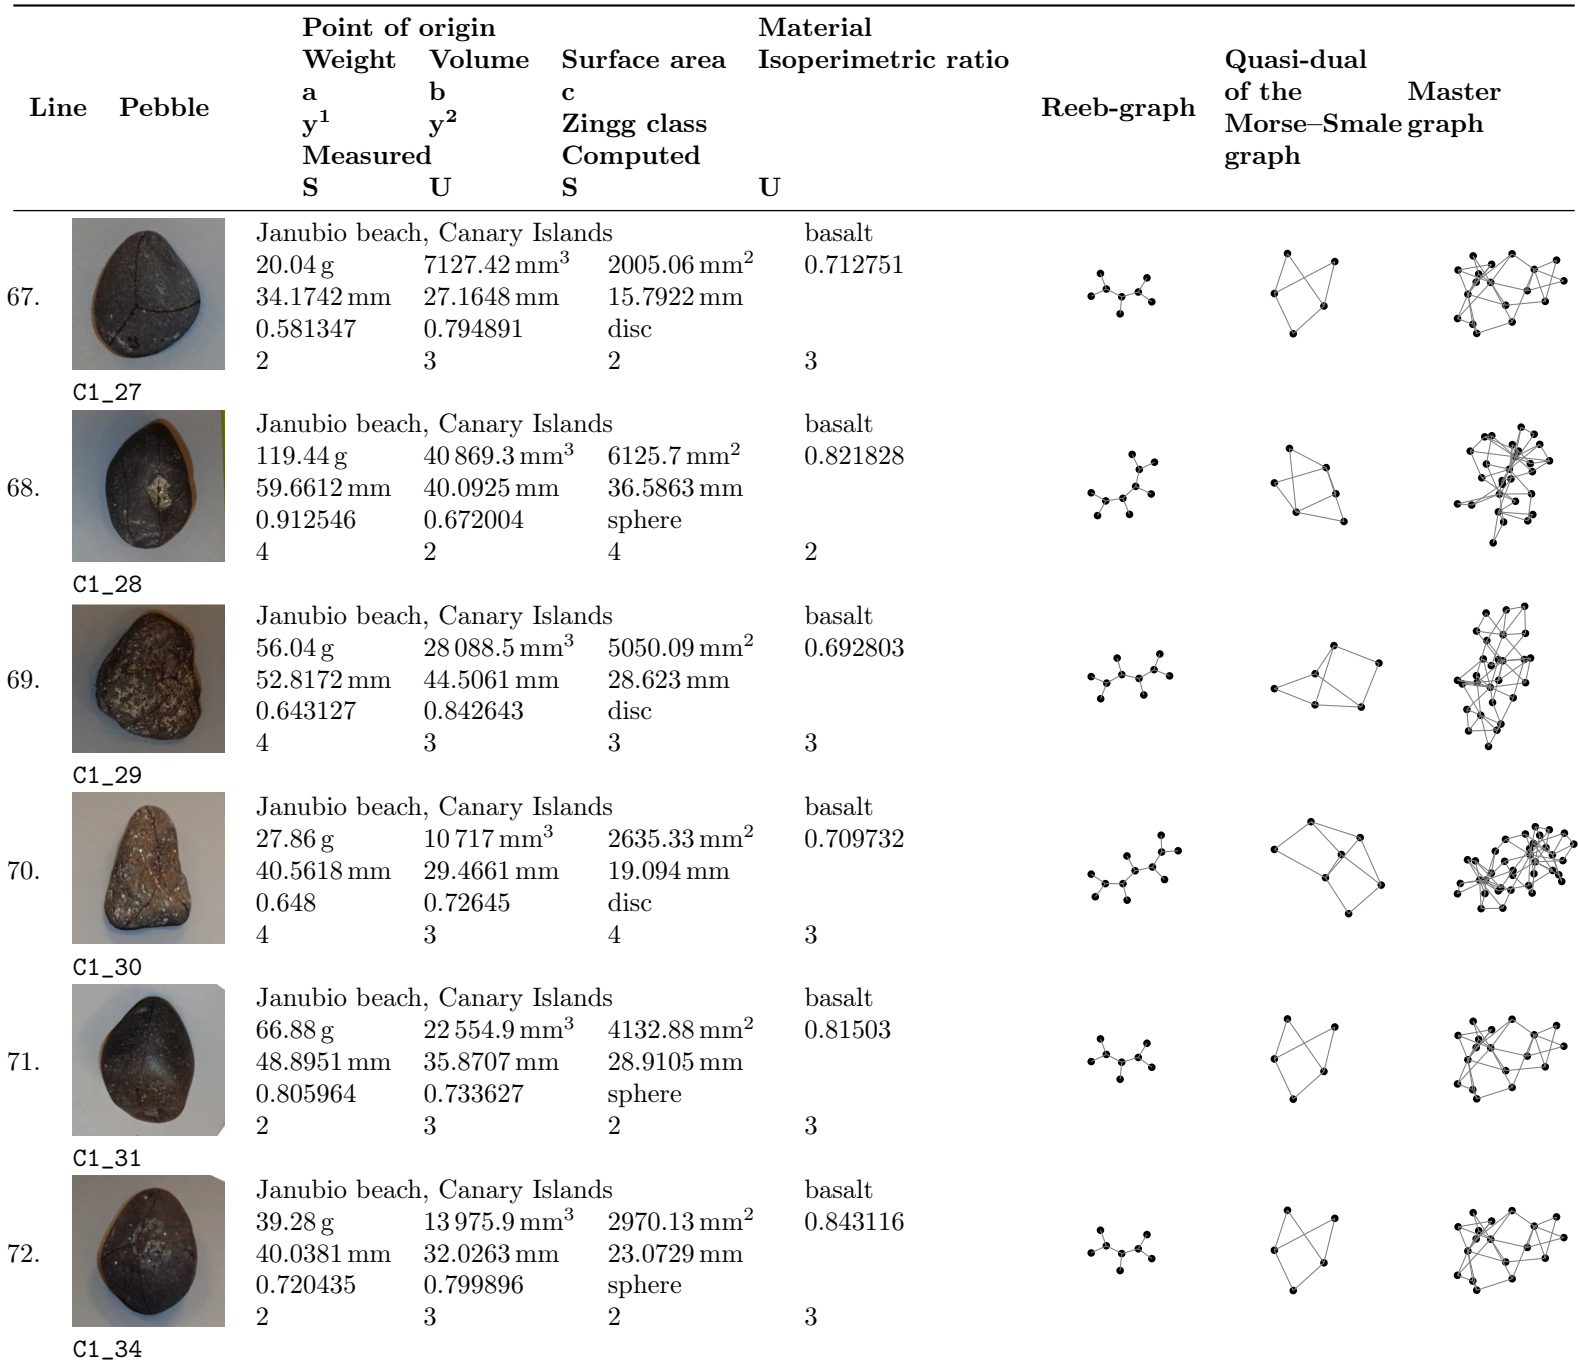 | Janubio beach, Canary Islands |                          |                         | basalt   | 0.843116            | 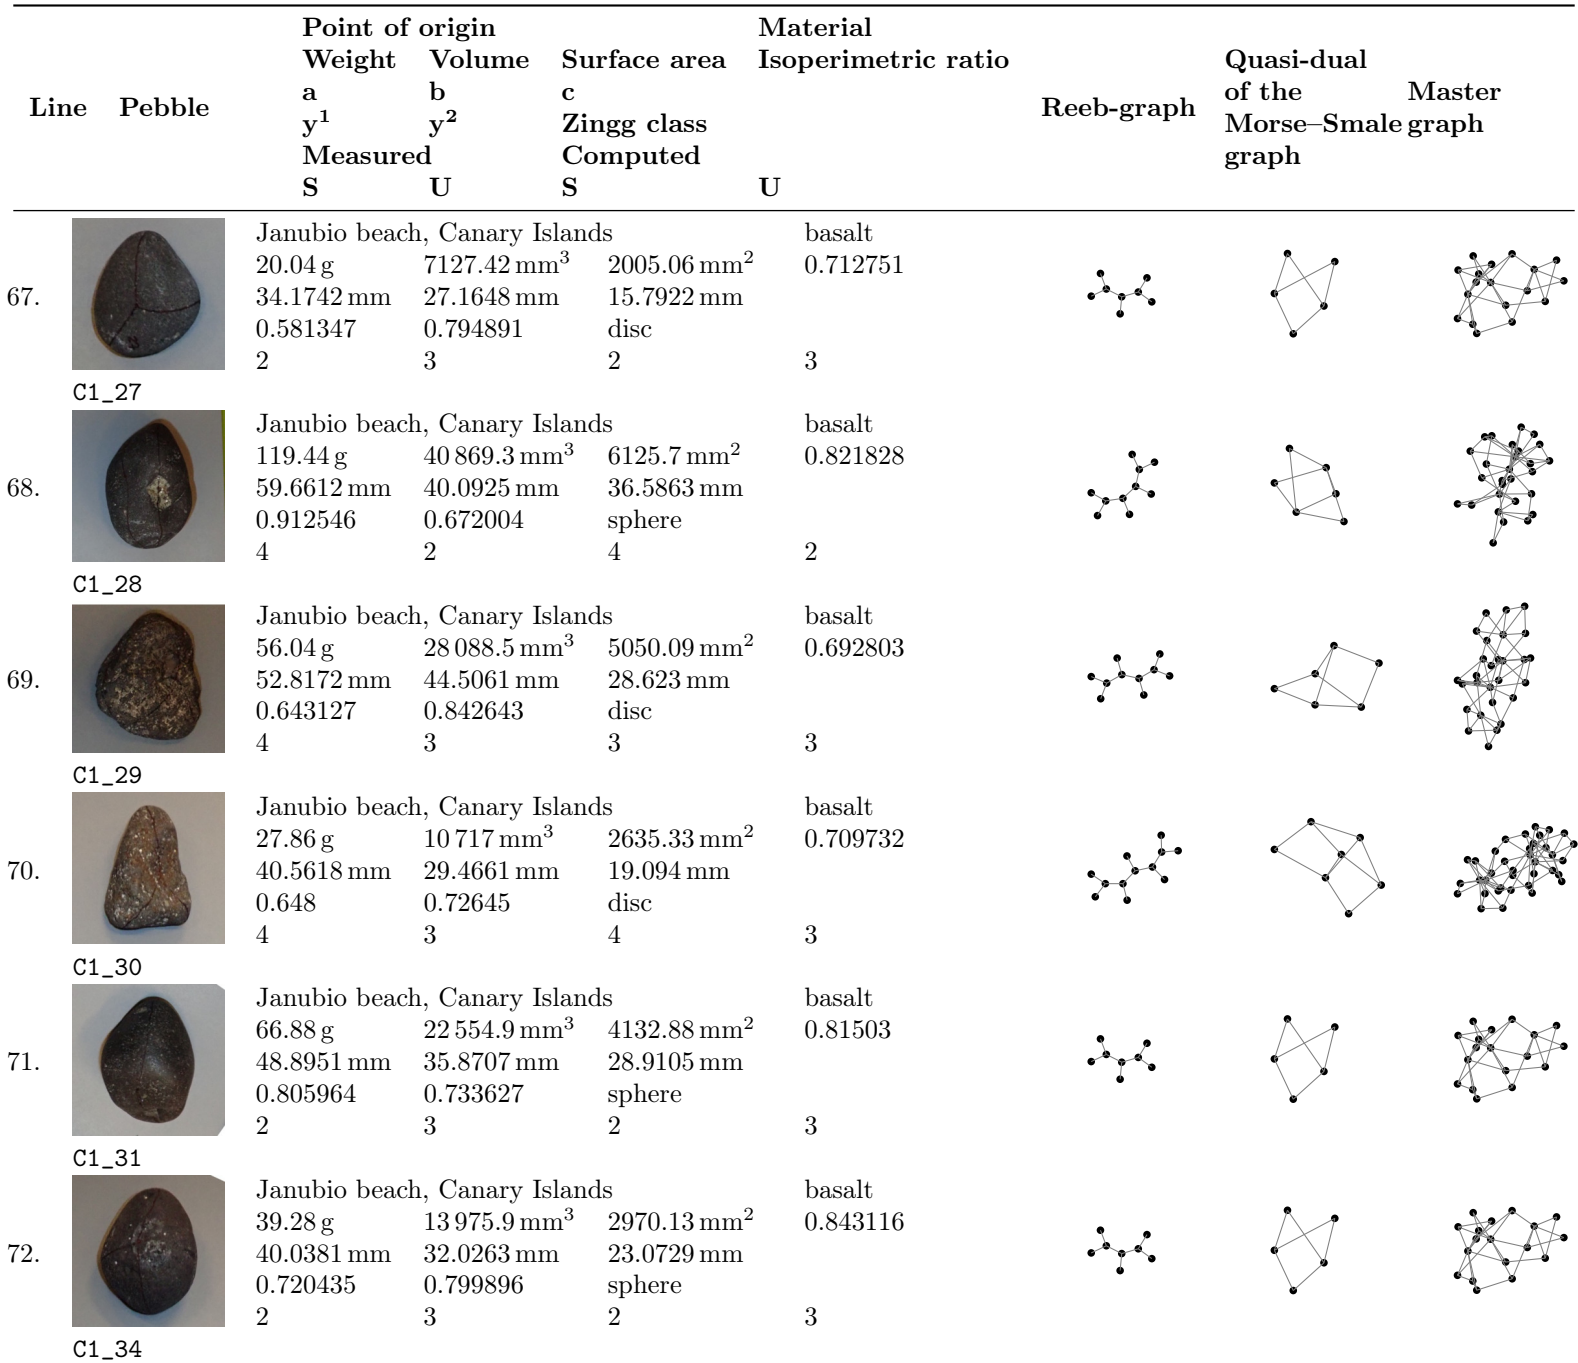 | 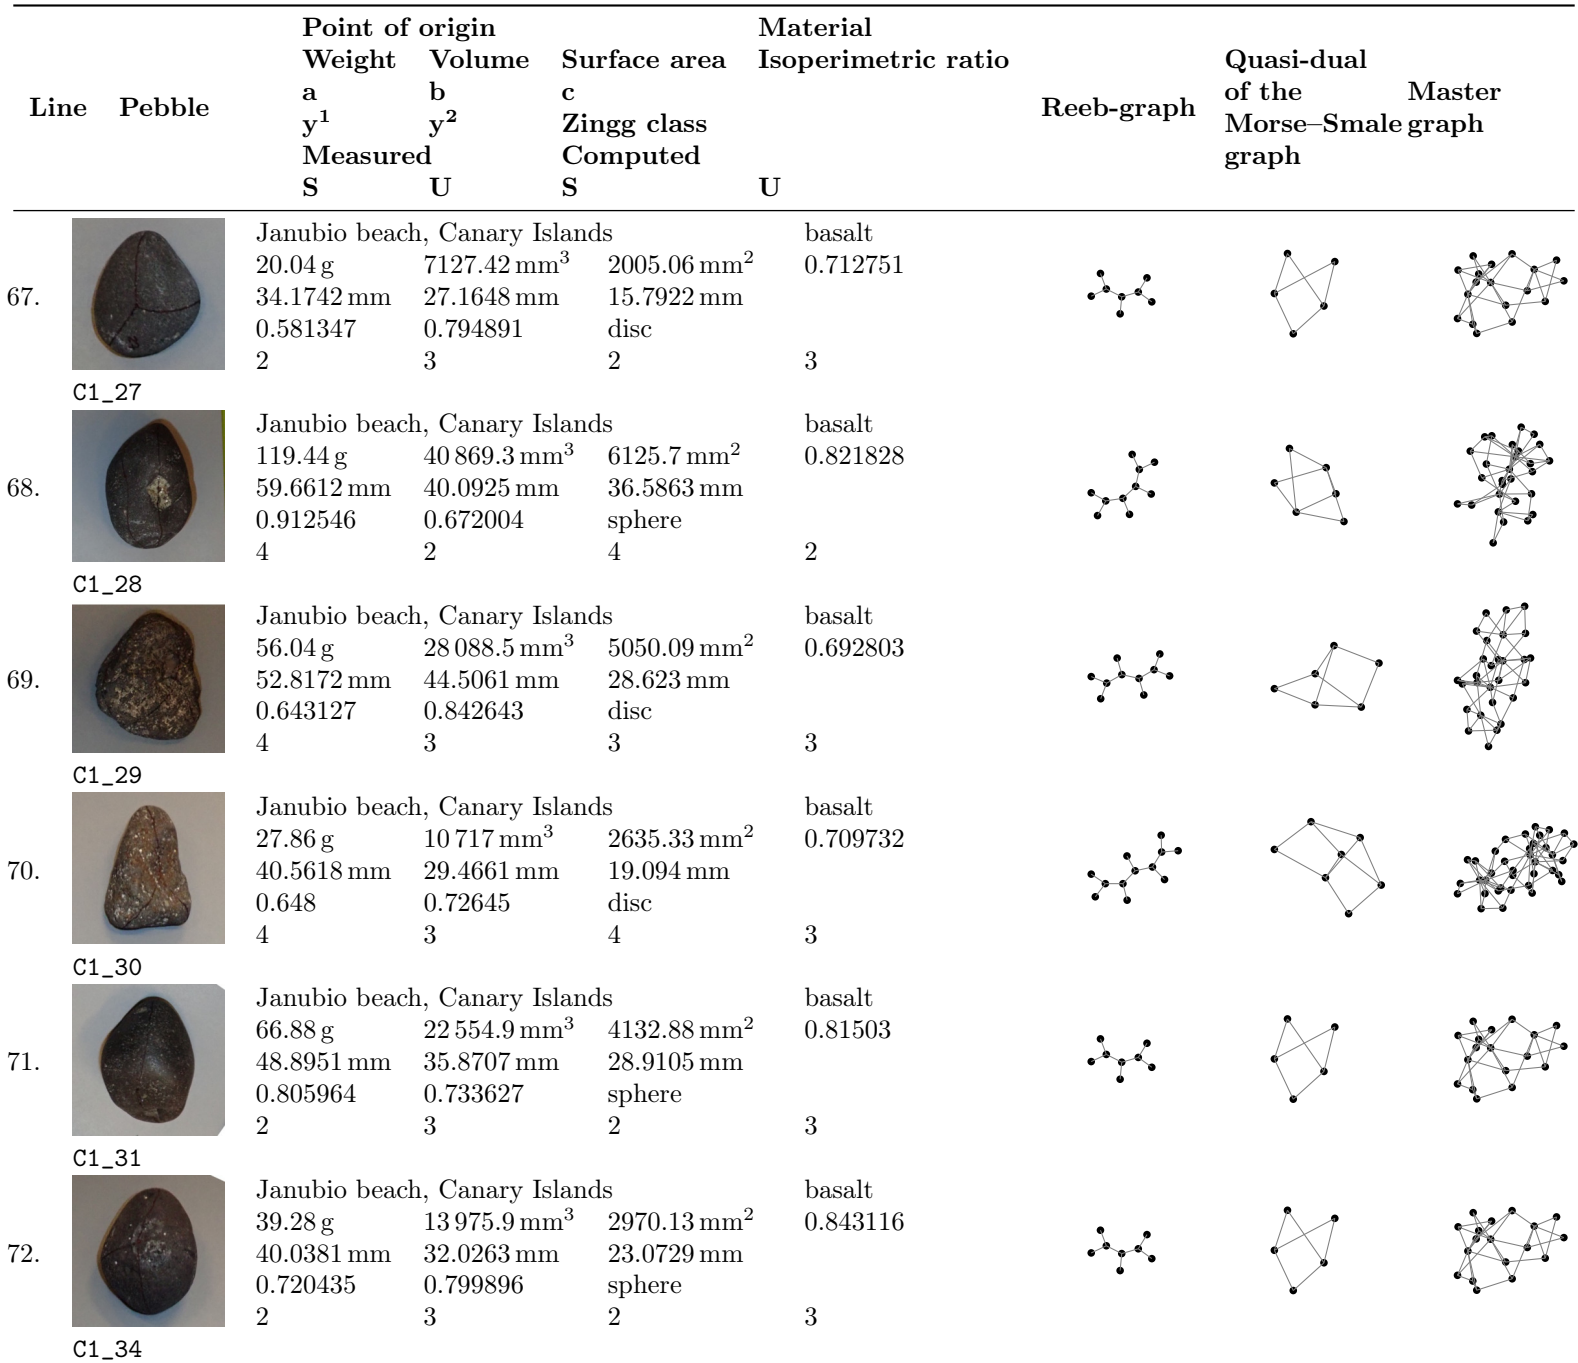 | 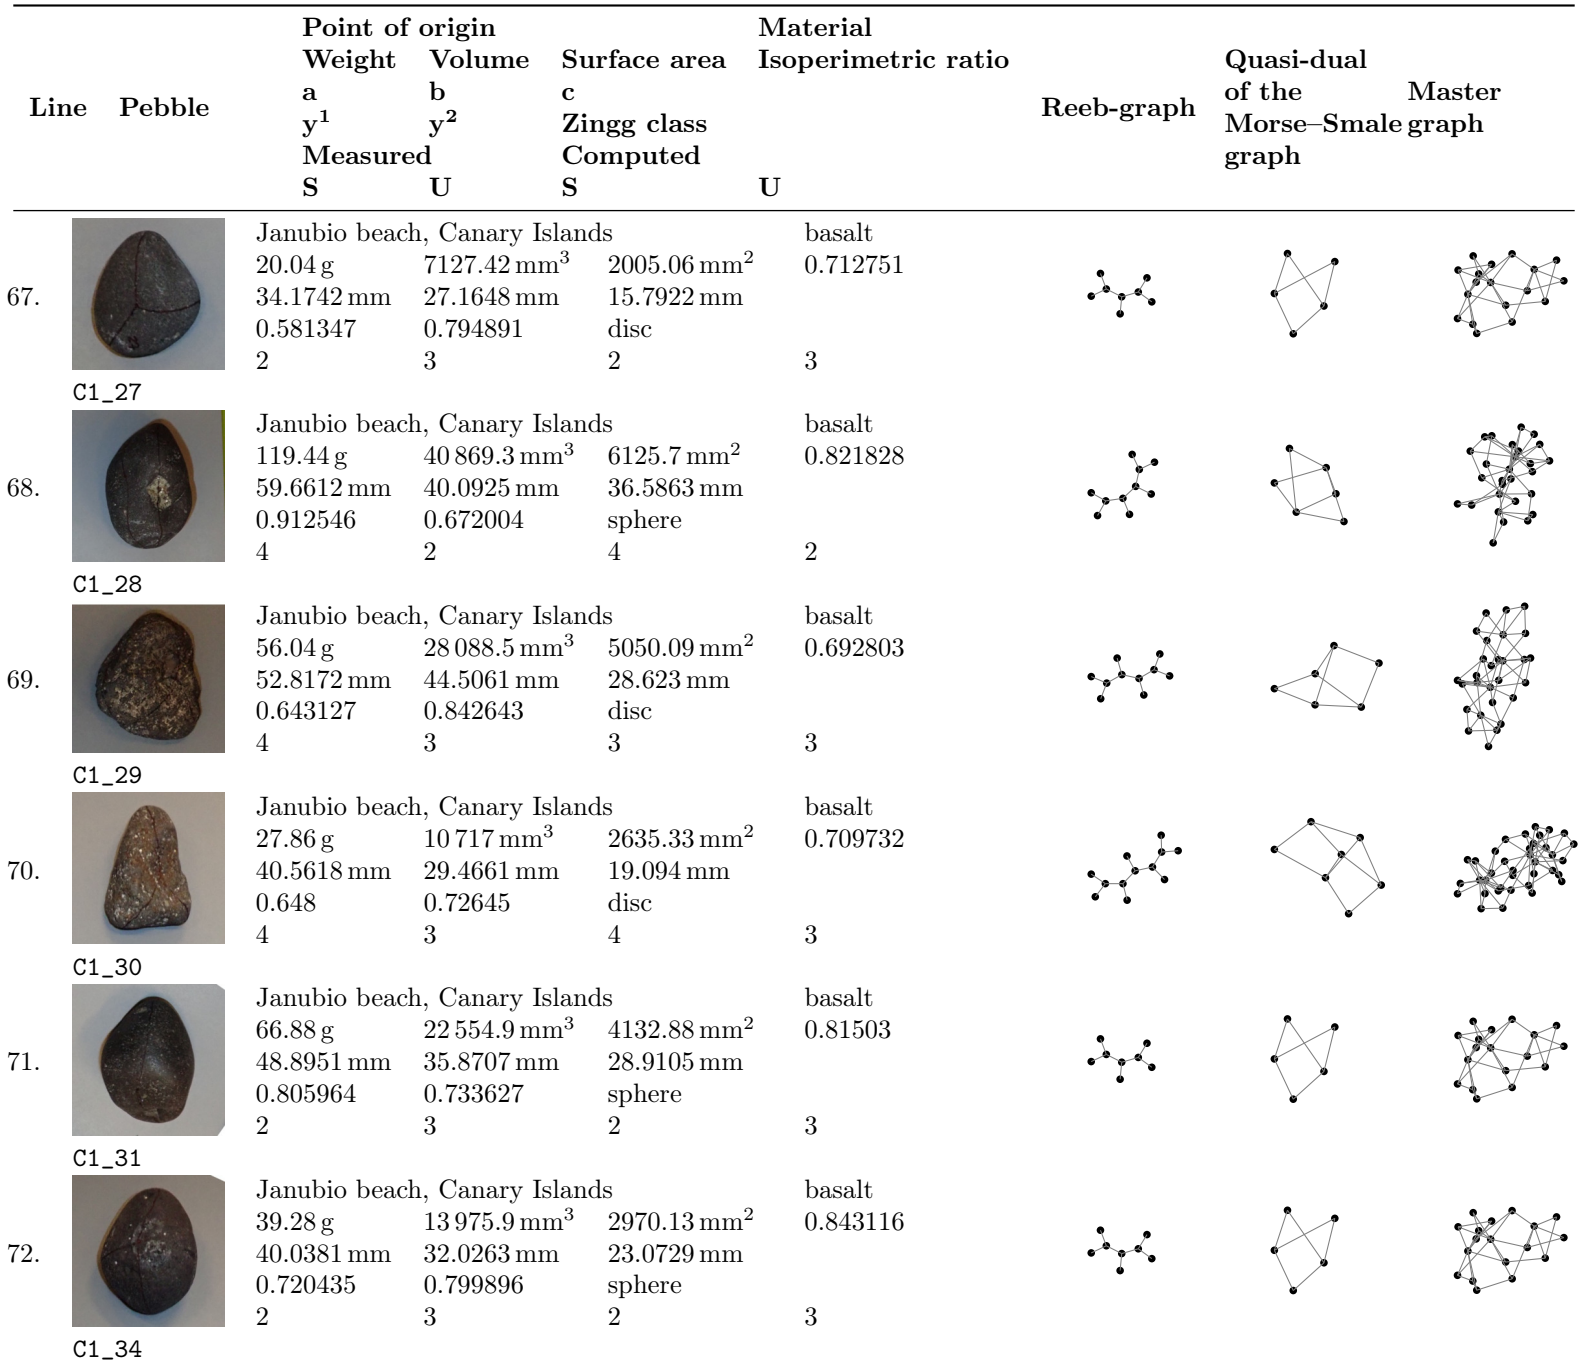 |
|      |                                                                                     | 39.28 g                       | 13 975.9 mm <sup>3</sup> | 2970.13 mm <sup>2</sup> |          |                     |                                                                                       |                                                                                       |                                                                                       |
|      |                                                                                     | 40.0381 mm                    | 32.0263 mm               | 23.0729 mm              |          |                     |                                                                                       |                                                                                       |                                                                                       |
|      |                                                                                     | 0.720435                      | 0.799896                 | sphere                  |          |                     |                                                                                       |                                                                                       |                                                                                       |
|      |                                                                                     | 2                             | 3                        | 2                       |          |                     |                                                                                       |                                                                                       |                                                                                       |
|      | C1_34                                                                               |                               |                          |                         |          |                     |                                                                                       |                                                                                       |                                                                                       |

| Line | Pebble                                                                              | Point of origin               |                          | Surface area            | Material            | Reeb-graph                                                                            | Quasi-dual<br>of the<br>Morse–Smale<br>graph                                          | Master                                                                                |
|------|-------------------------------------------------------------------------------------|-------------------------------|--------------------------|-------------------------|---------------------|---------------------------------------------------------------------------------------|---------------------------------------------------------------------------------------|---------------------------------------------------------------------------------------|
|      |                                                                                     | Weight                        | Volume                   |                         |                     |                                                                                       |                                                                                       |                                                                                       |
|      |                                                                                     | a                             | b                        |                         |                     |                                                                                       |                                                                                       |                                                                                       |
|      |                                                                                     | y <sup>1</sup>                | y <sup>2</sup>           | c                       | Isoperimetric ratio |                                                                                       |                                                                                       |                                                                                       |
|      |                                                                                     | Measured                      |                          | Zingg class             |                     |                                                                                       |                                                                                       |                                                                                       |
|      |                                                                                     | S                             | U                        | Computed                | U                   |                                                                                       |                                                                                       |                                                                                       |
| 73.  | 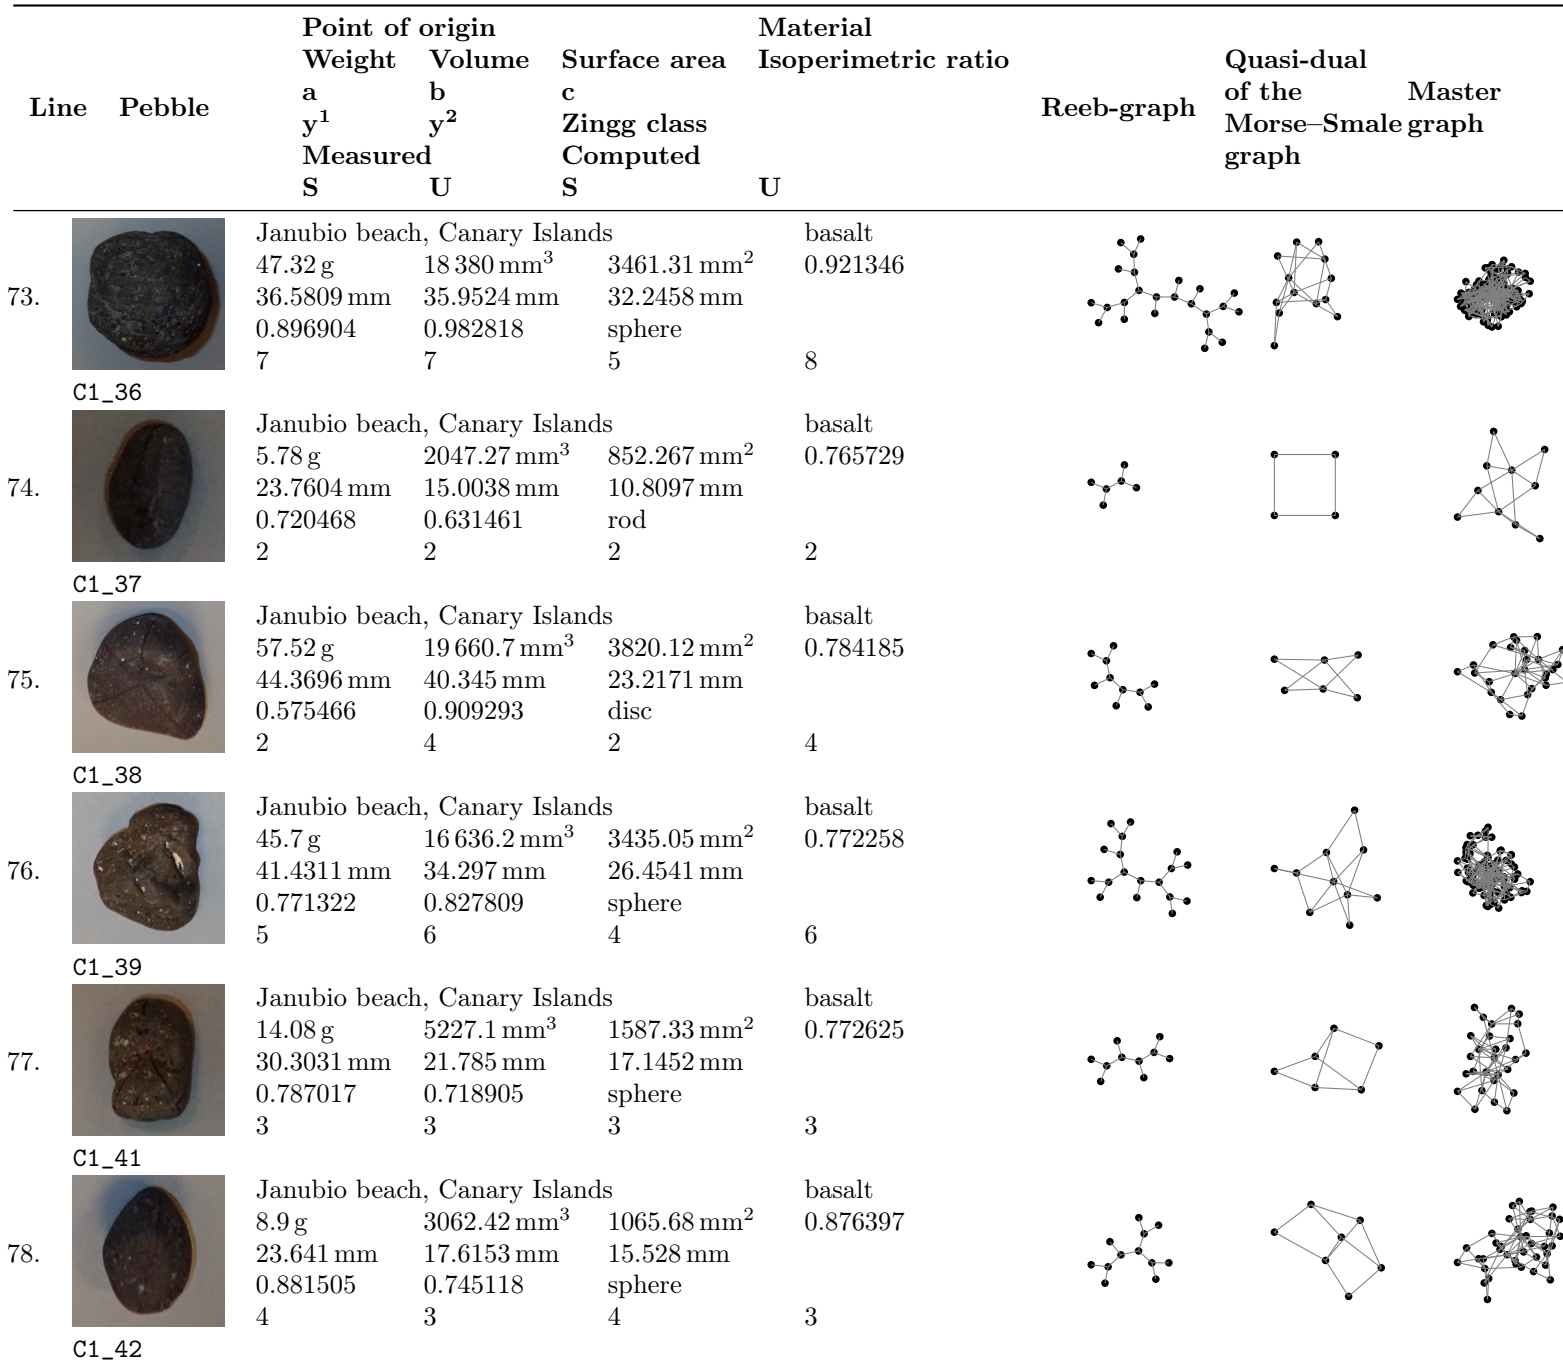   | Janubio beach, Canary Islands |                          |                         | basalt              | 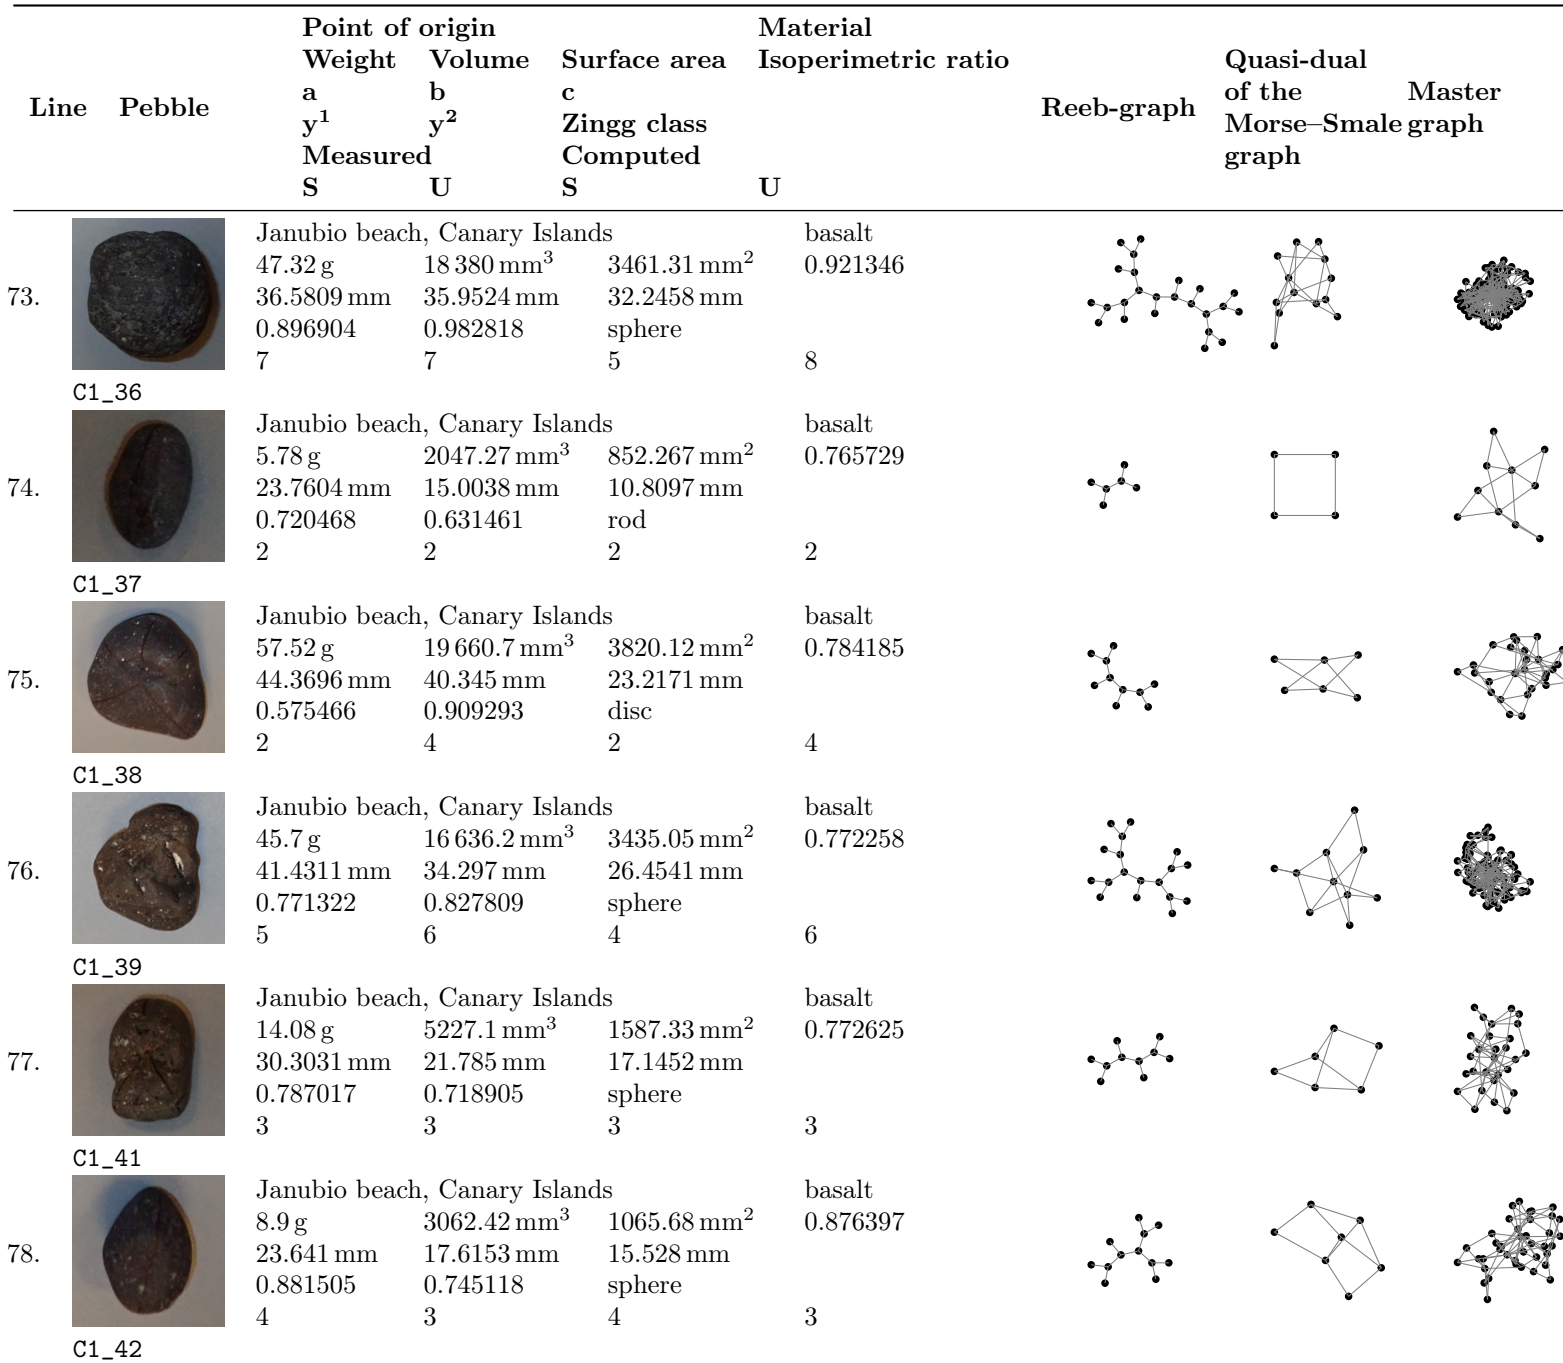   | 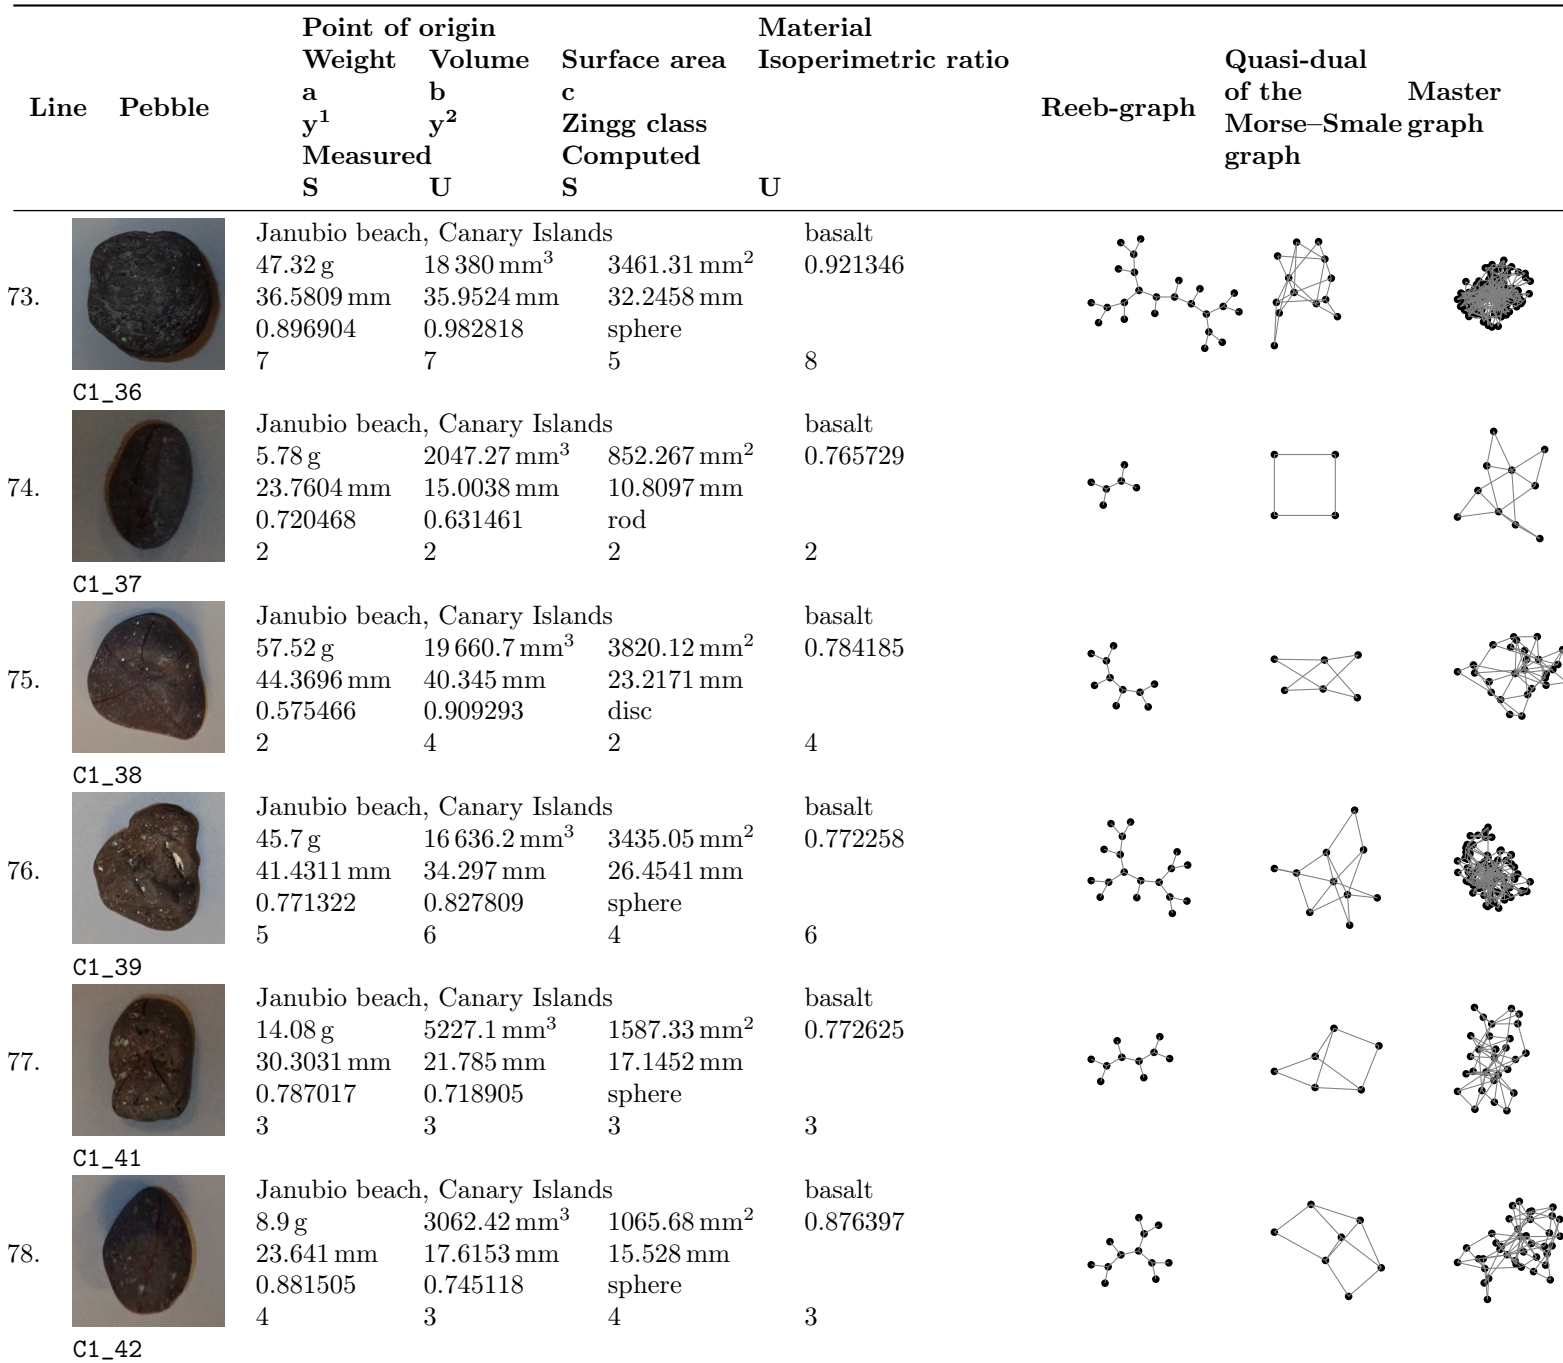   | 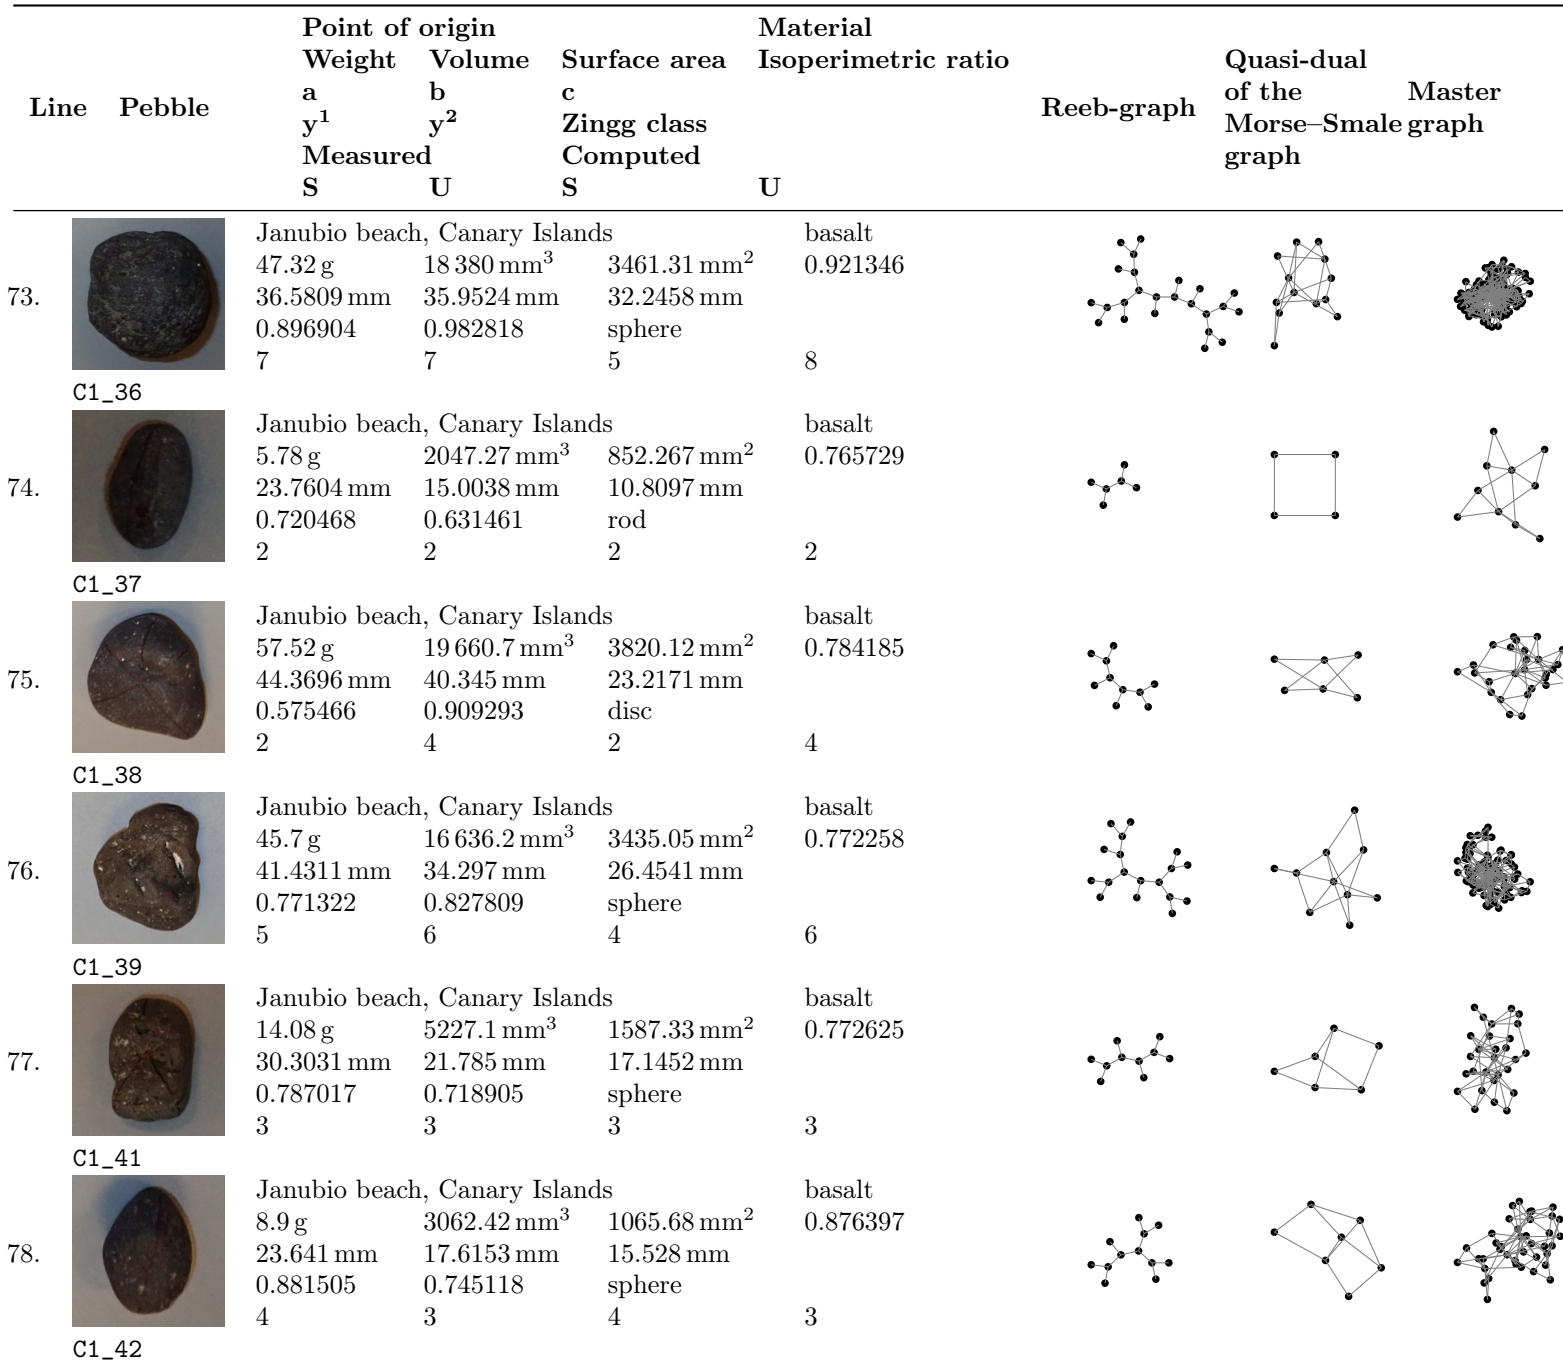   |
|      |                                                                                     | 47.32 g                       | 18 380 mm <sup>3</sup>   | 3461.31 mm <sup>2</sup> | 0.921346            |                                                                                       |                                                                                       |                                                                                       |
|      |                                                                                     | 36.5809 mm                    | 35.9524 mm               | 32.2458 mm              |                     |                                                                                       |                                                                                       |                                                                                       |
|      |                                                                                     | 0.896904                      | 0.982818                 | sphere                  |                     |                                                                                       |                                                                                       |                                                                                       |
|      |                                                                                     | 7                             | 7                        | 5                       | 8                   |                                                                                       |                                                                                       |                                                                                       |
|      |                                                                                     | C1_36                         |                          |                         |                     |                                                                                       |                                                                                       |                                                                                       |
| 74.  | 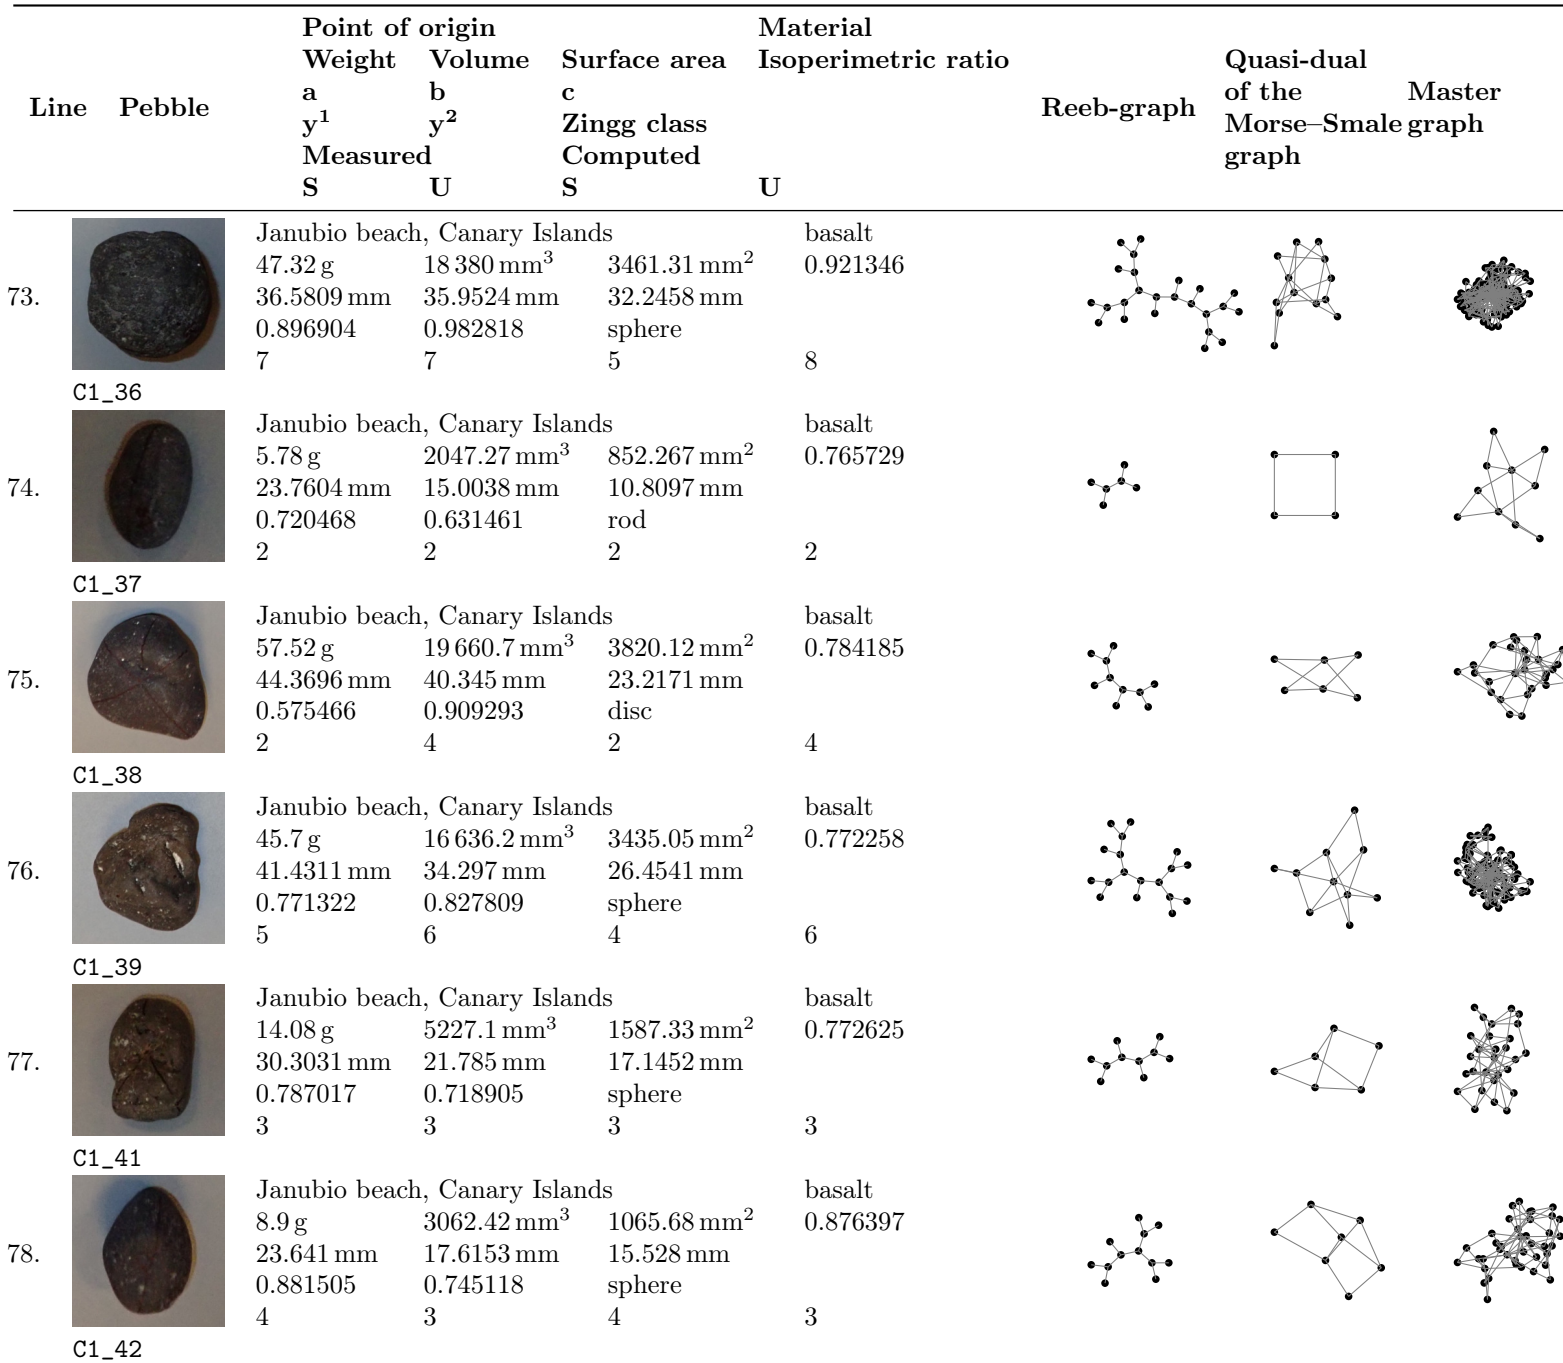   | Janubio beach, Canary Islands |                          |                         | basalt              | 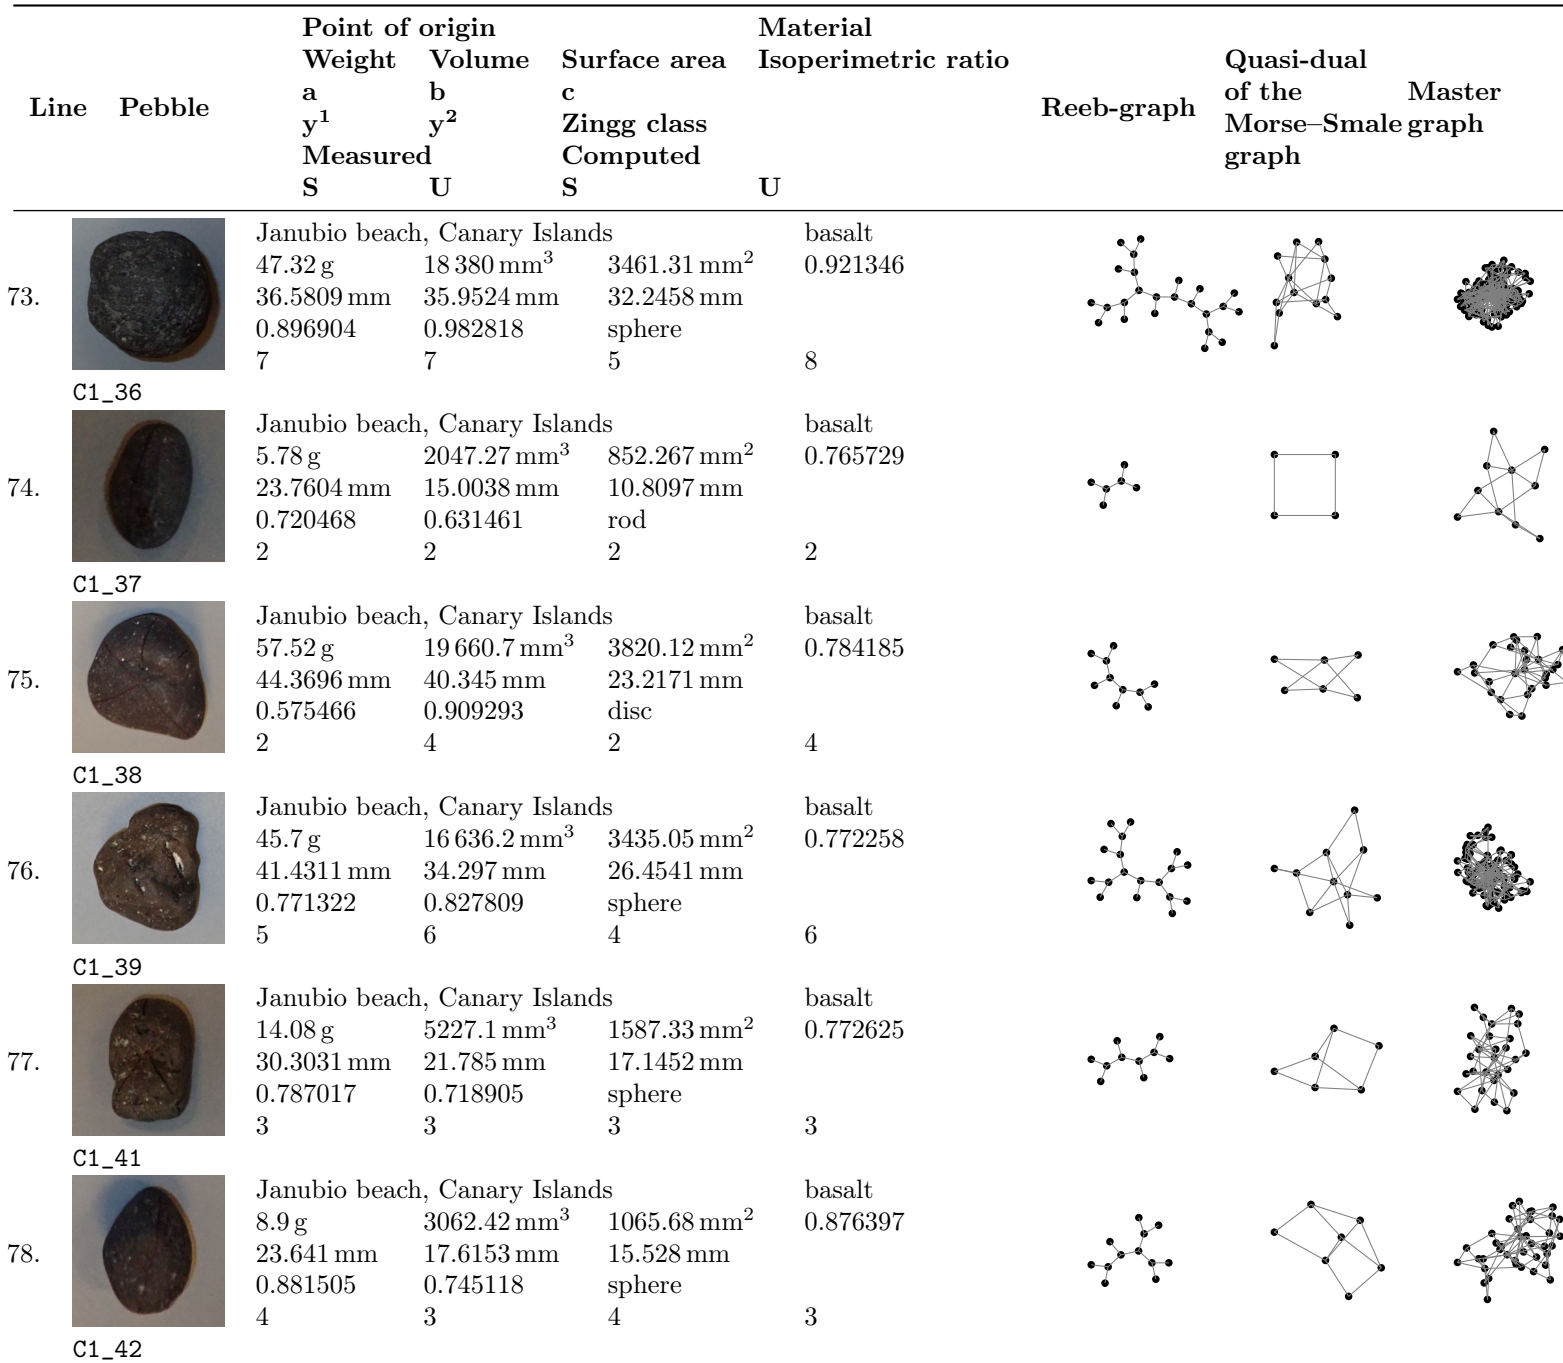   | 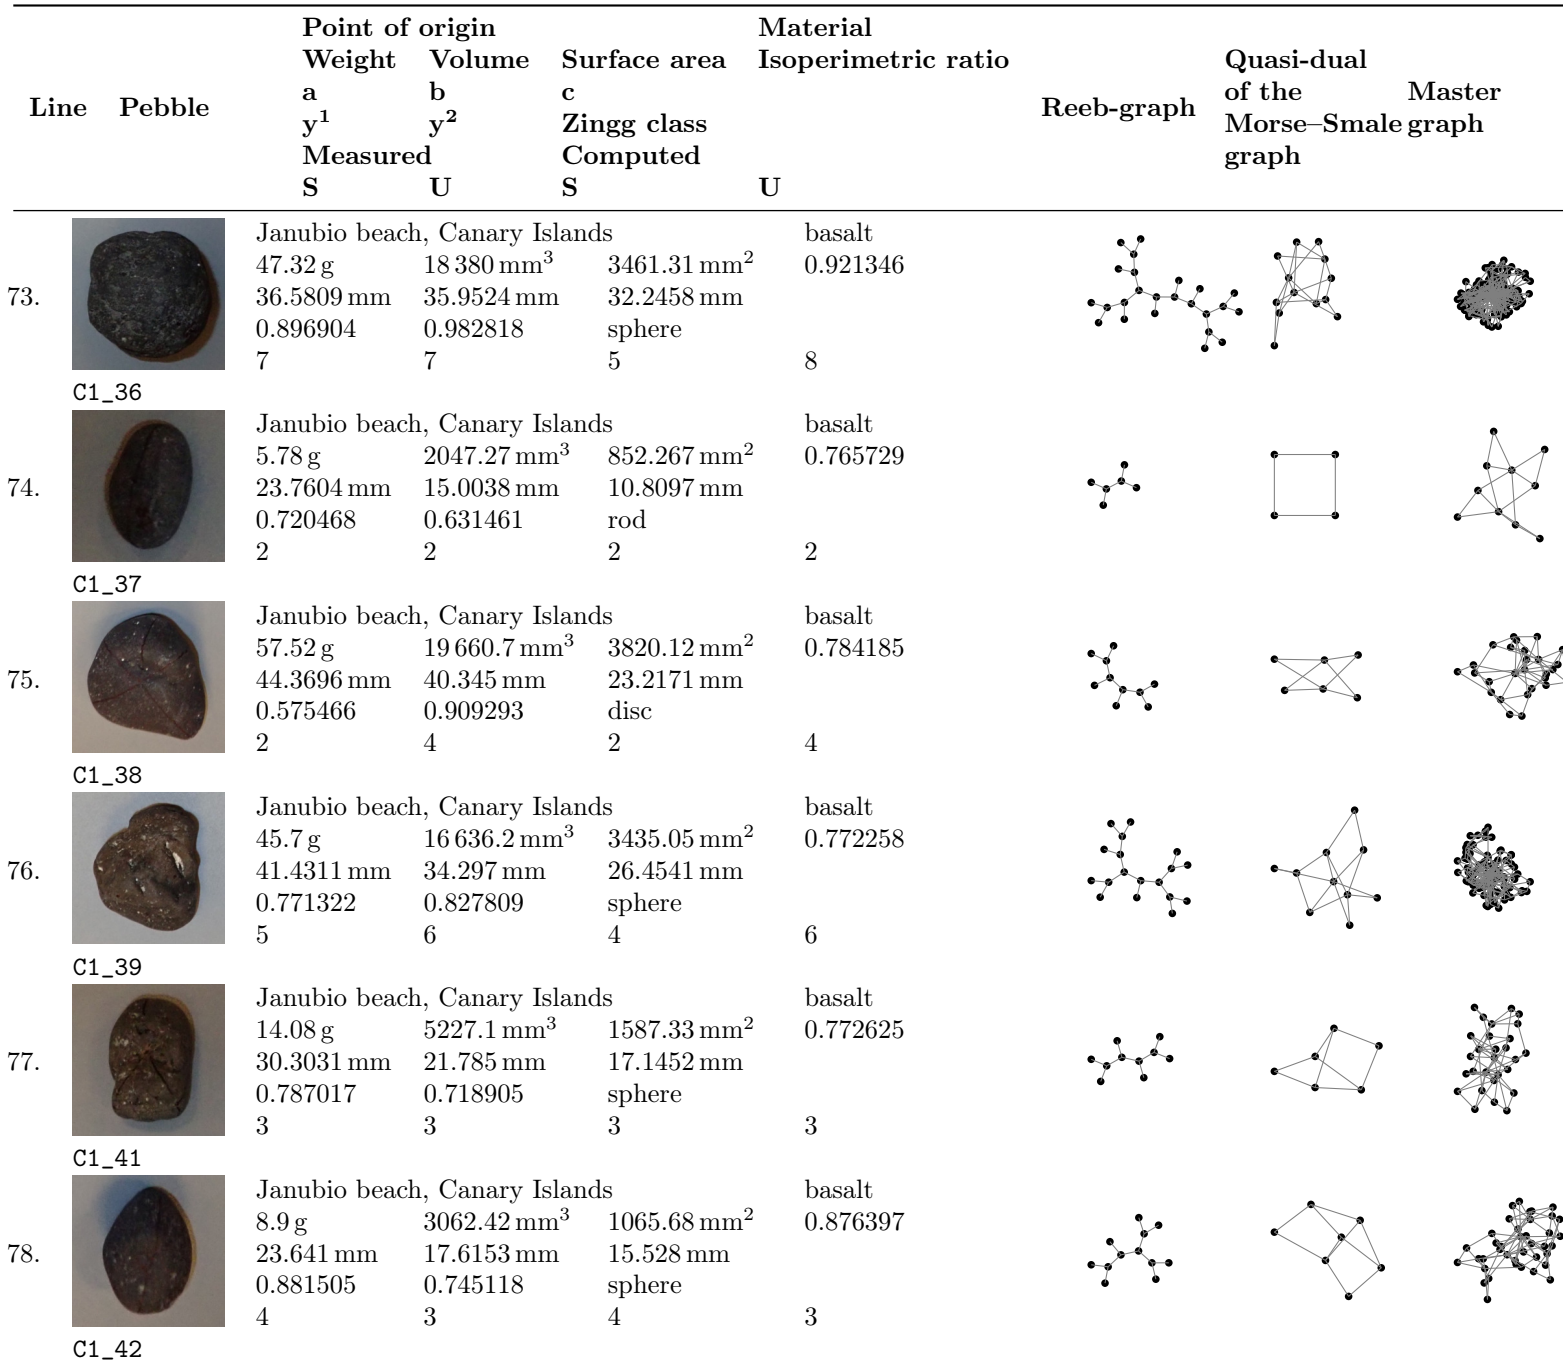   | 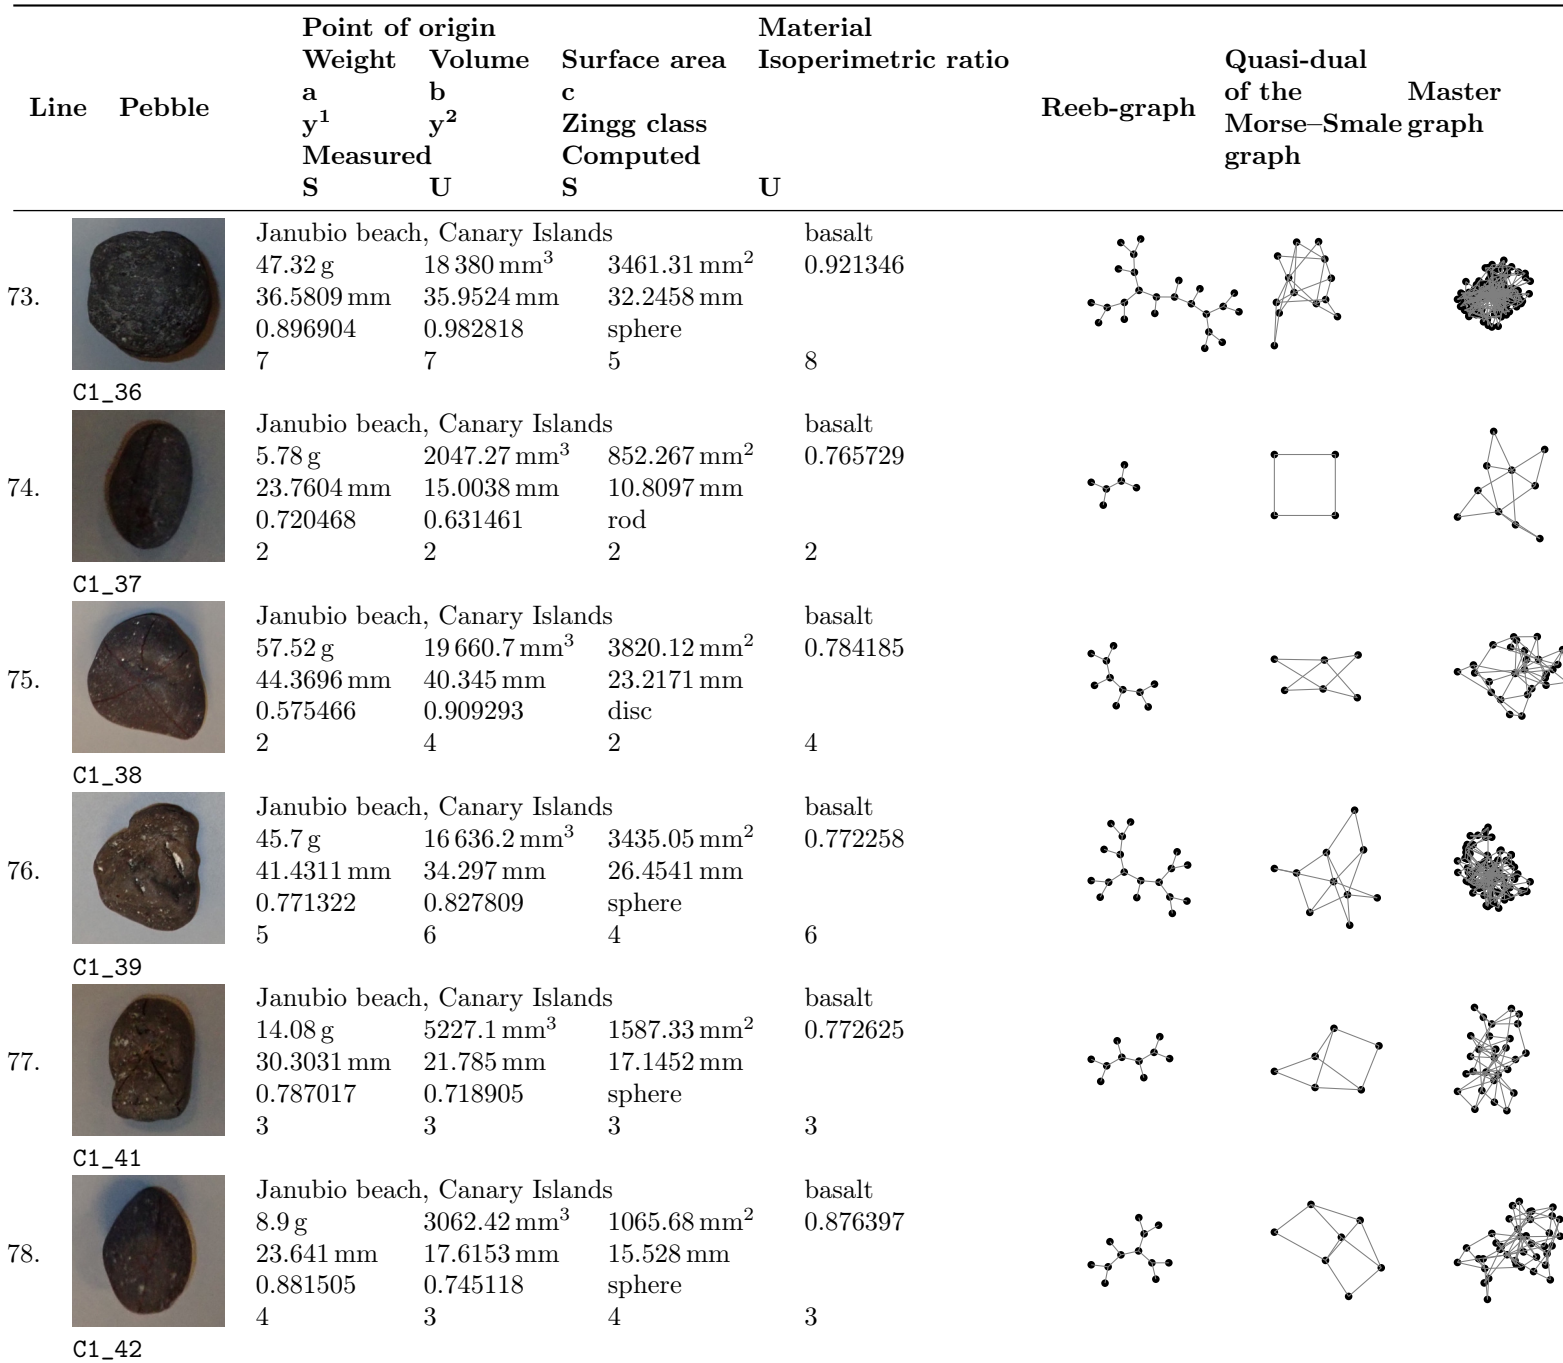   |
|      |                                                                                     | 5.78 g                        | 2047.27 mm <sup>3</sup>  | 852.267 mm <sup>2</sup> | 0.765729            |                                                                                       |                                                                                       |                                                                                       |
|      |                                                                                     | 23.7604 mm                    | 15.0038 mm               | 10.8097 mm              |                     |                                                                                       |                                                                                       |                                                                                       |
|      |                                                                                     | 0.720468                      | 0.631461                 | rod                     |                     |                                                                                       |                                                                                       |                                                                                       |
|      |                                                                                     | 2                             | 2                        | 2                       | 2                   |                                                                                       |                                                                                       |                                                                                       |
|      |                                                                                     | C1_37                         |                          |                         |                     |                                                                                       |                                                                                       |                                                                                       |
| 75.  | 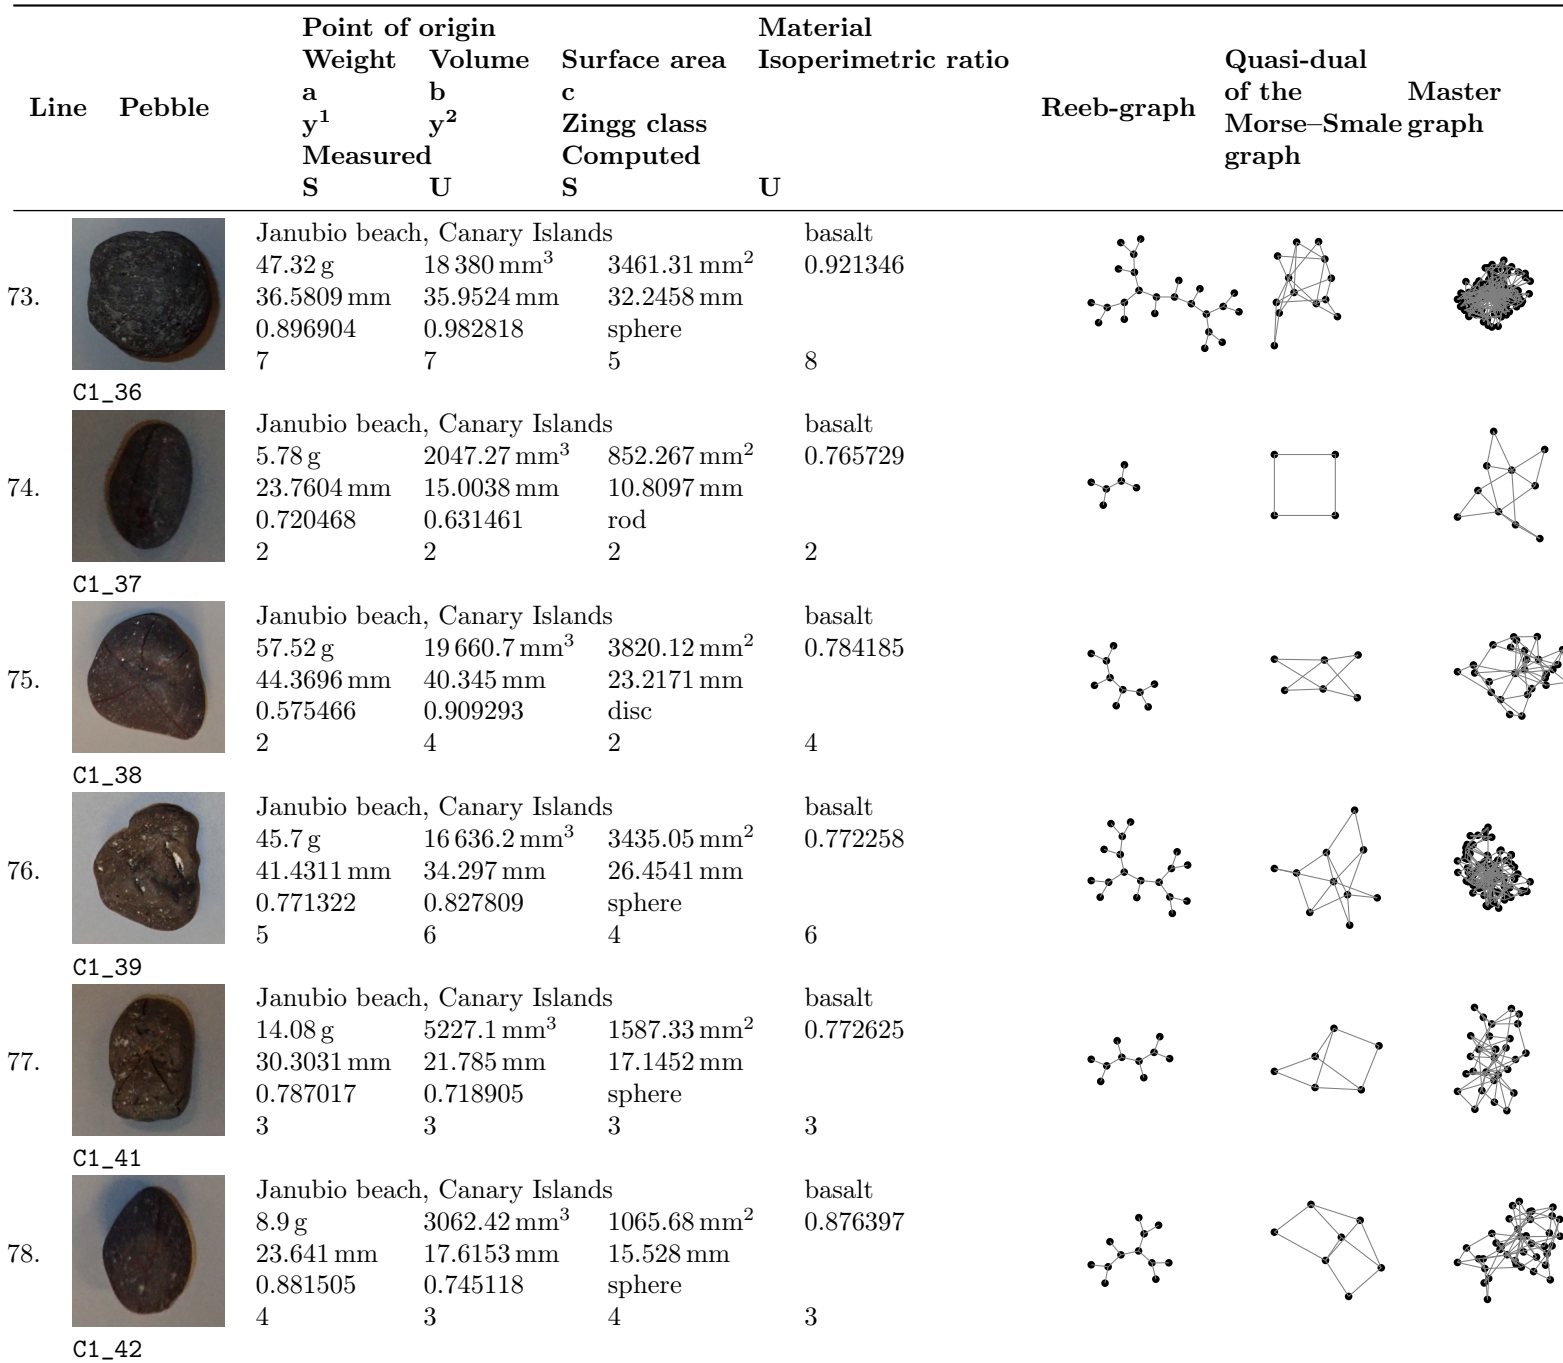   | Janubio beach, Canary Islands |                          |                         | basalt              | 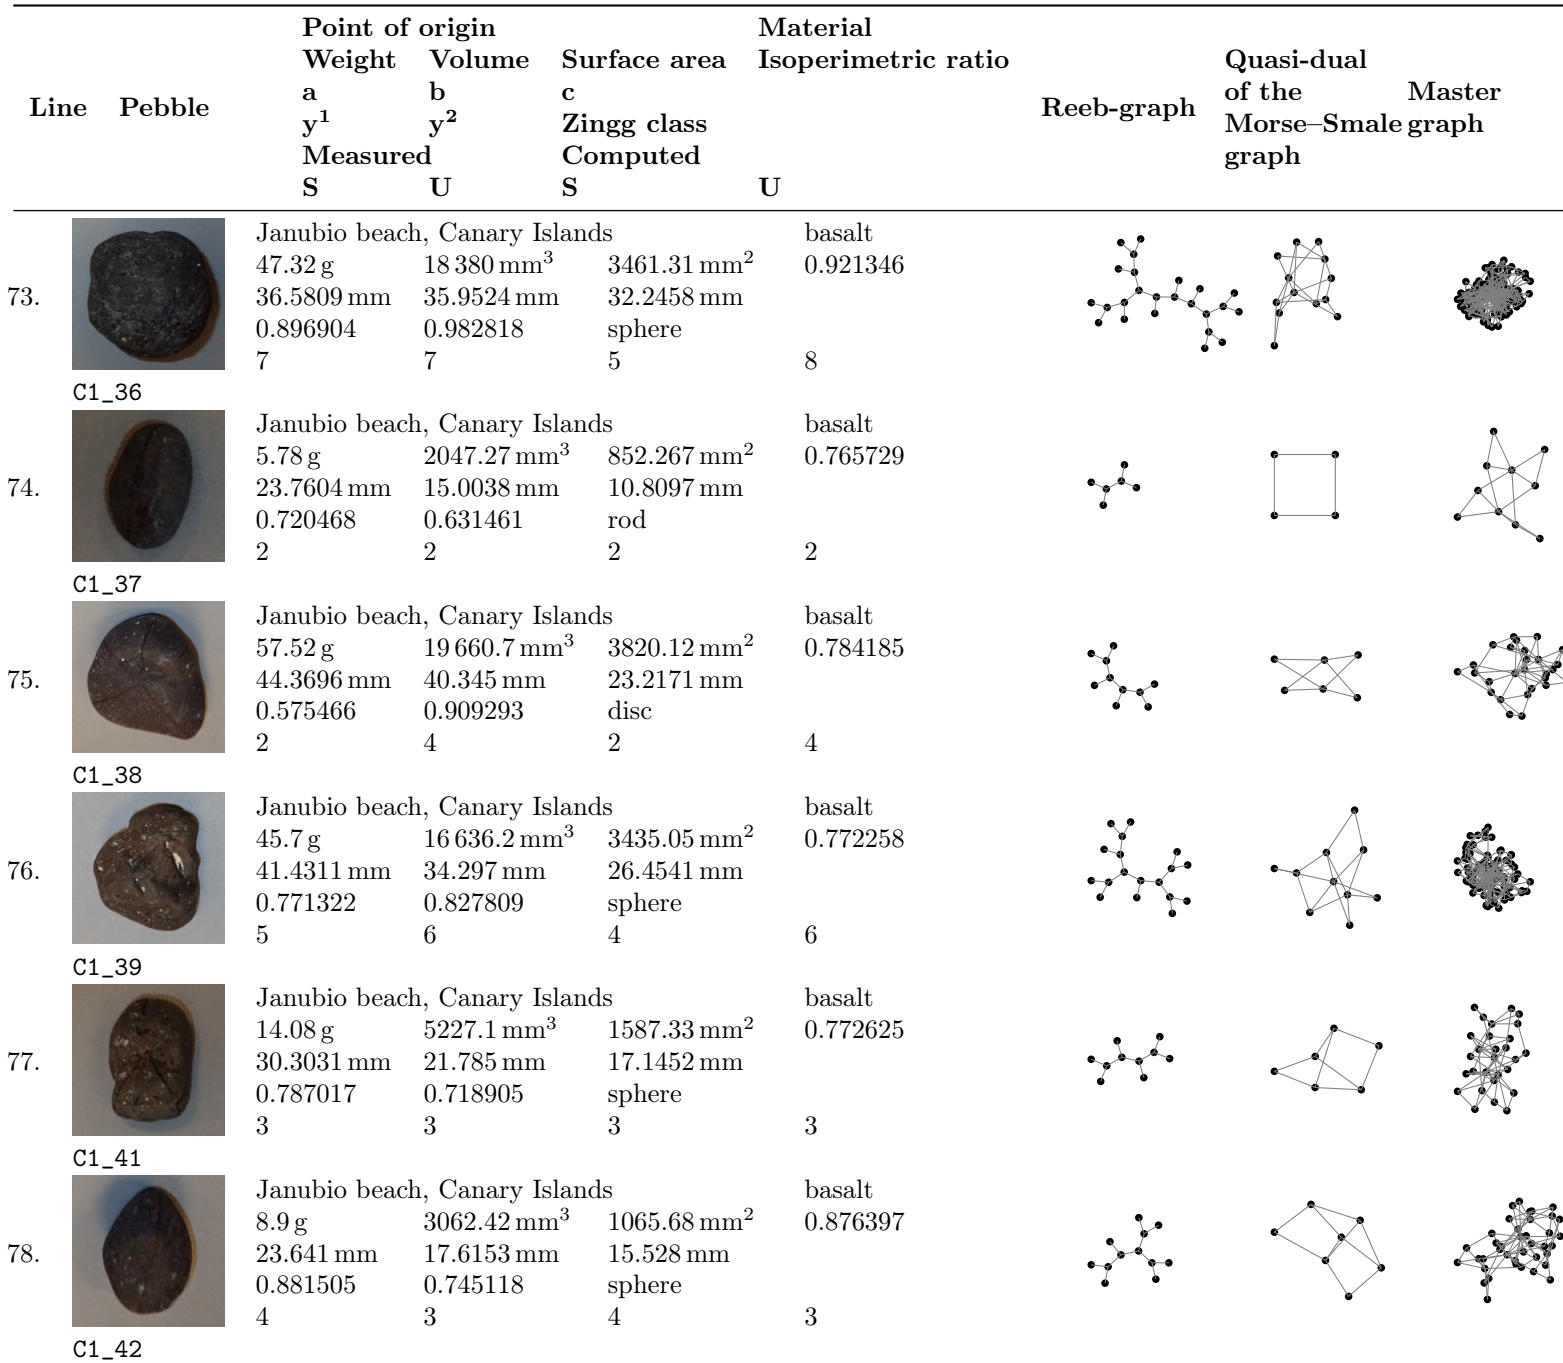   | 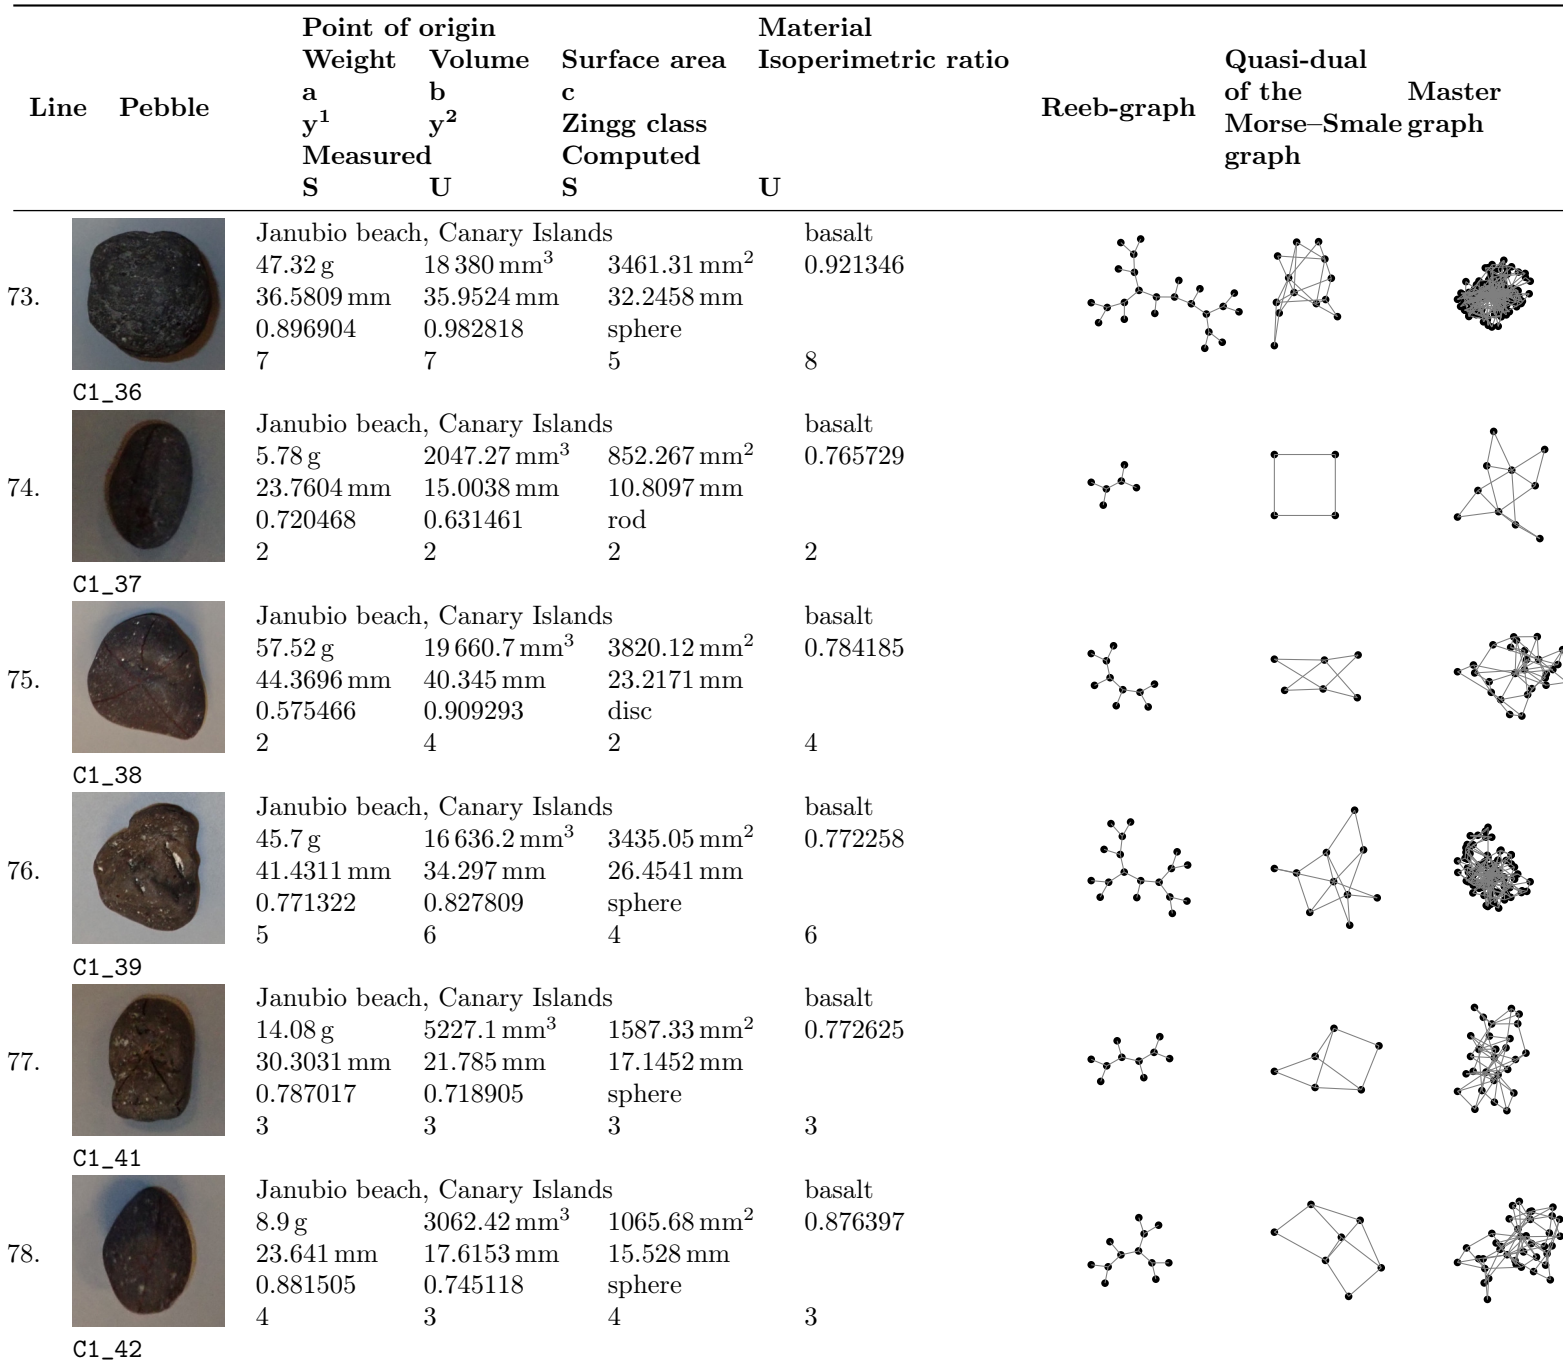   | 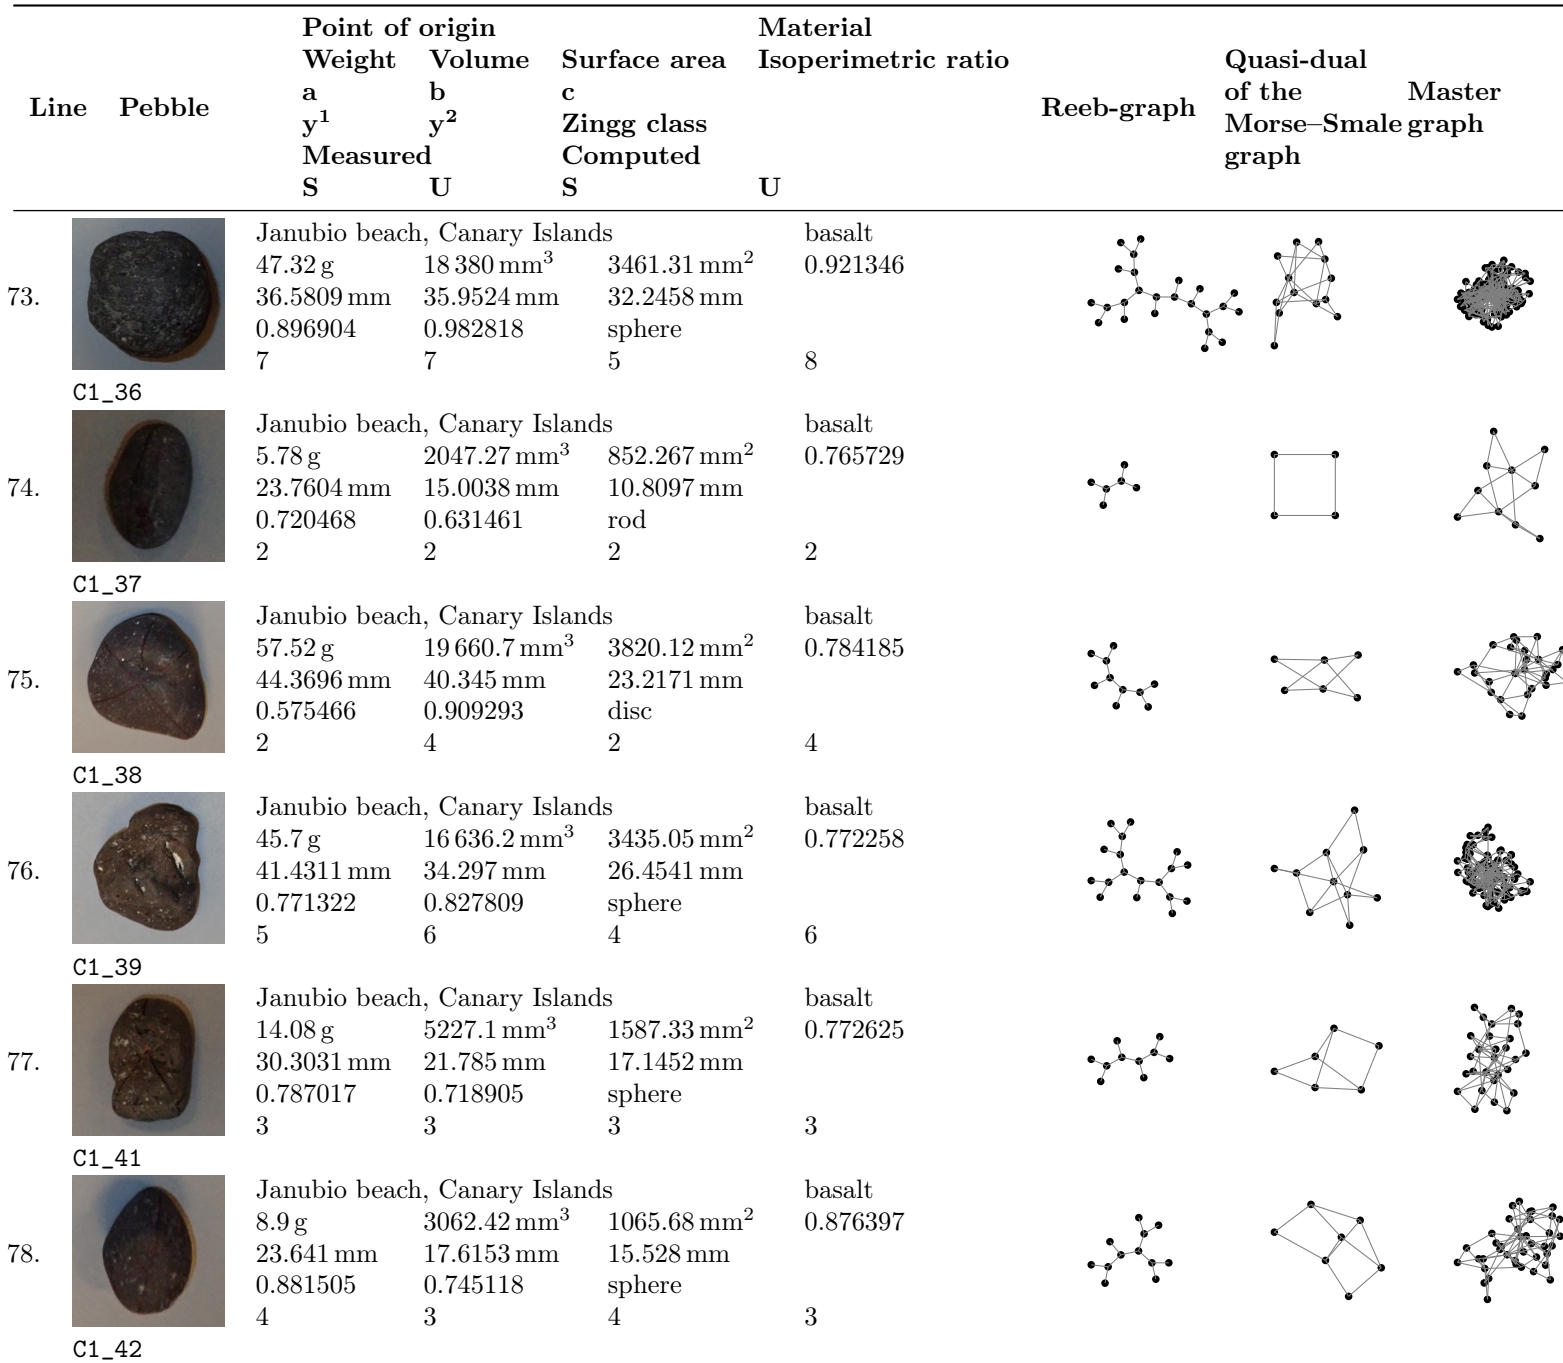   |
|      |                                                                                     | 57.52 g                       | 19 660.7 mm <sup>3</sup> | 3820.12 mm <sup>2</sup> | 0.784185            |                                                                                       |                                                                                       |                                                                                       |
|      |                                                                                     | 44.3696 mm                    | 40.345 mm                | 23.2171 mm              |                     |                                                                                       |                                                                                       |                                                                                       |
|      |                                                                                     | 0.575466                      | 0.909293                 | disc                    |                     |                                                                                       |                                                                                       |                                                                                       |
|      |                                                                                     | 2                             | 4                        | 2                       | 4                   |                                                                                       |                                                                                       |                                                                                       |
|      |                                                                                     | C1_38                         |                          |                         |                     |                                                                                       |                                                                                       |                                                                                       |
| 76.  | 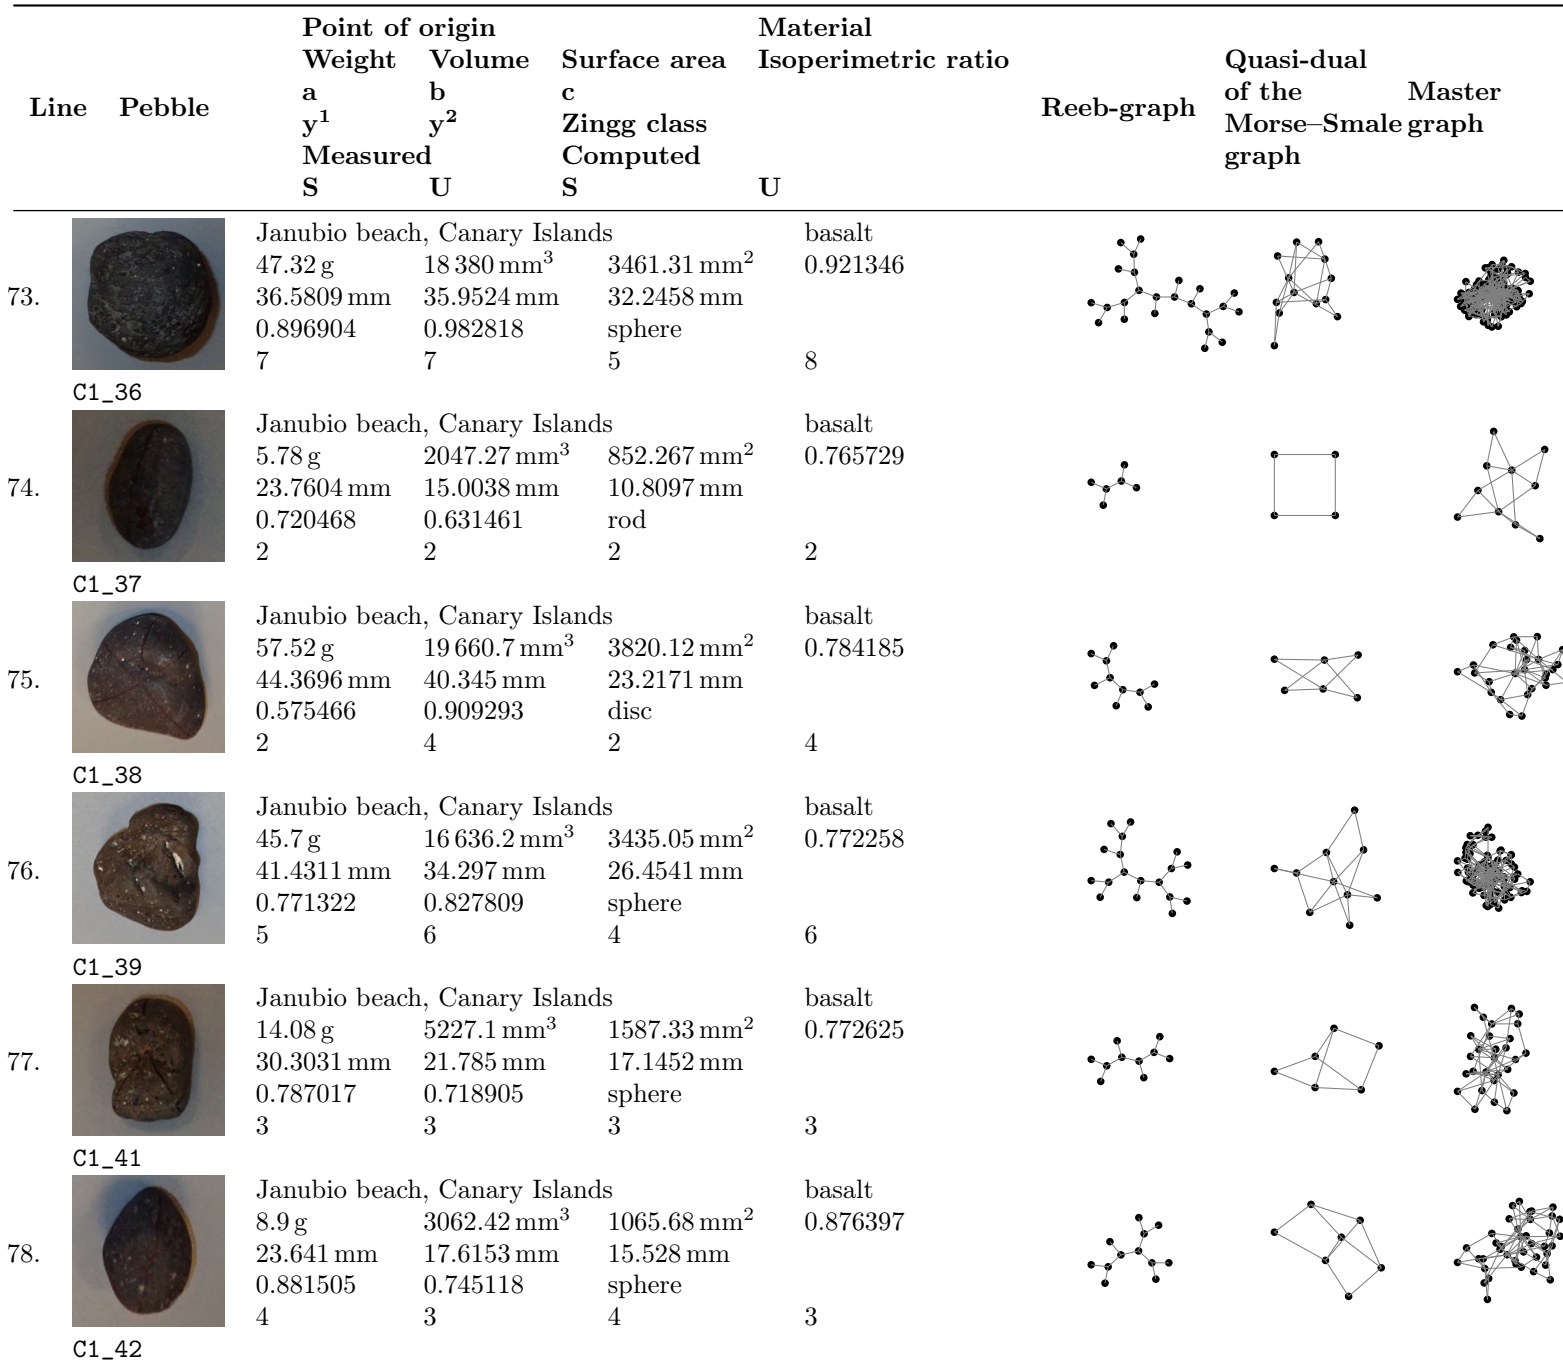  | Janubio beach, Canary Islands |                          |                         | basalt              | 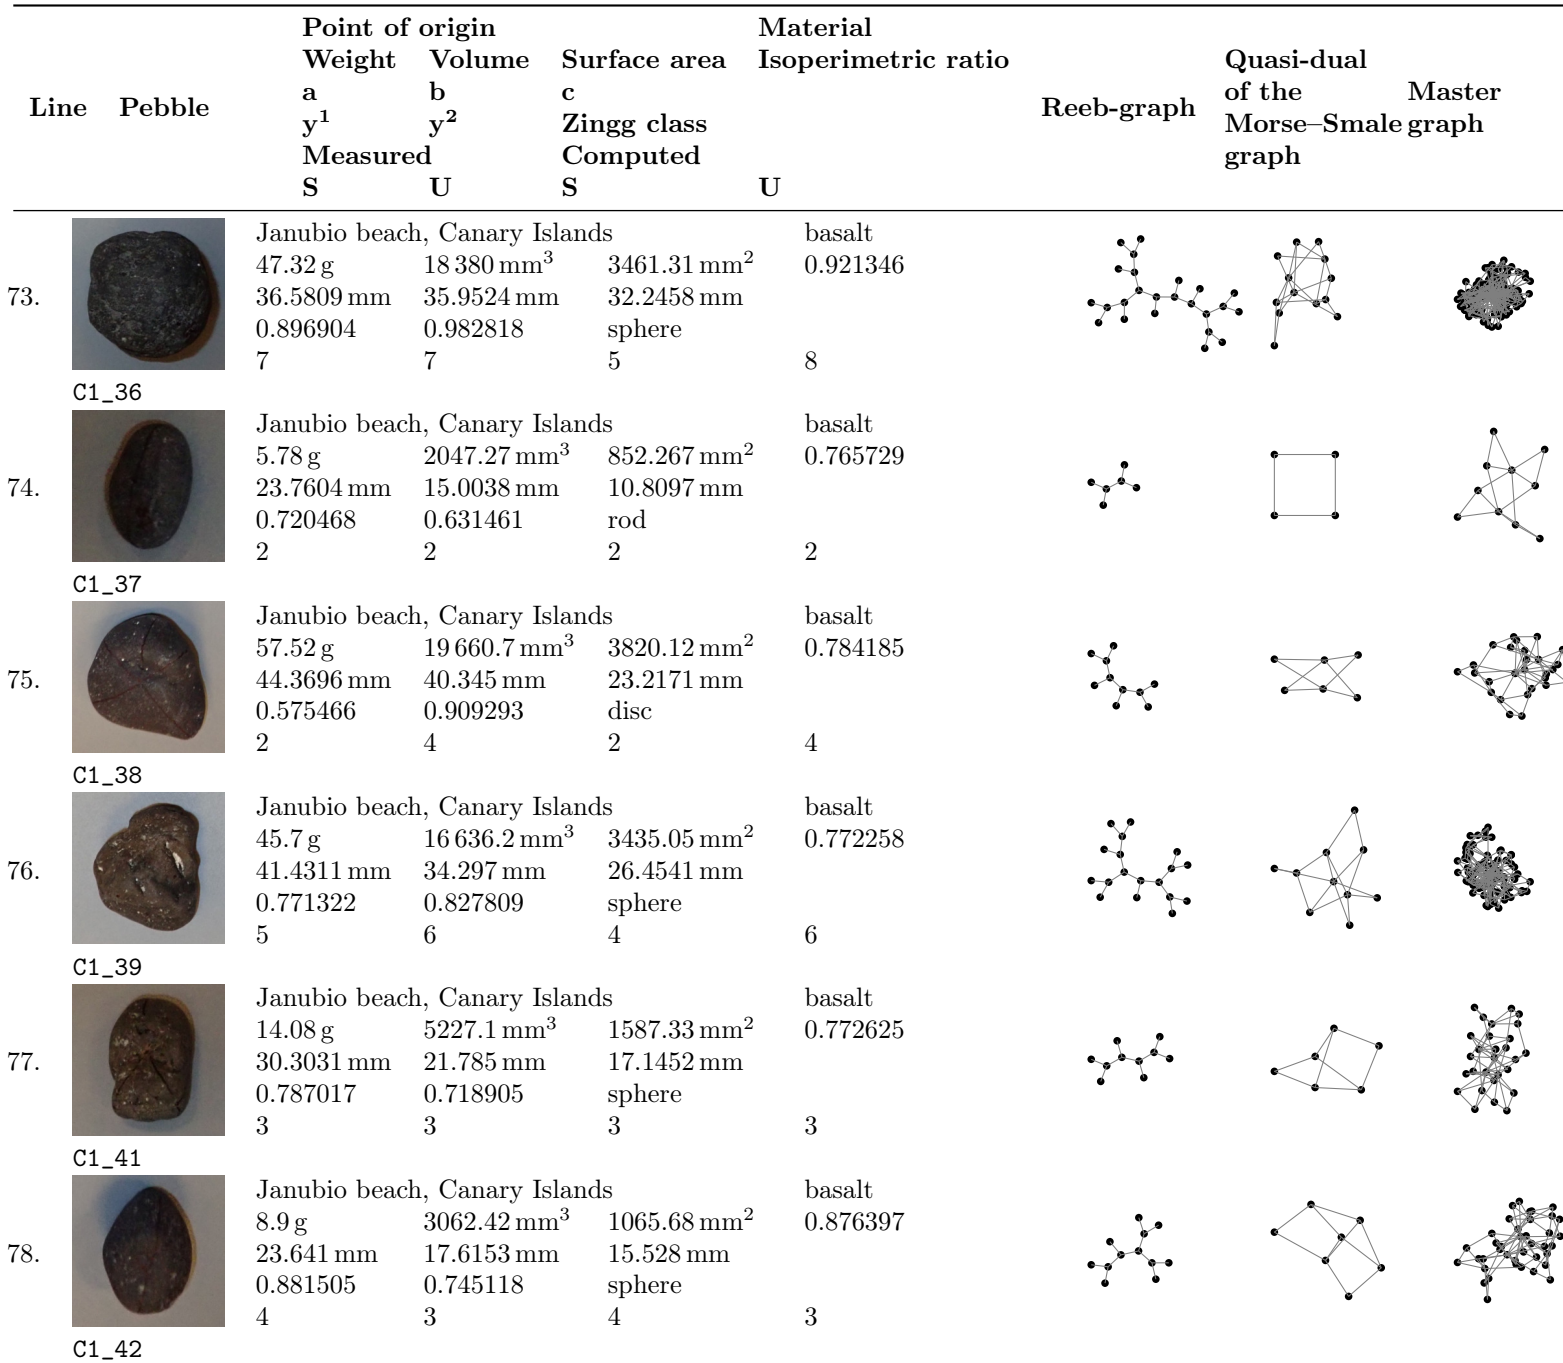  | 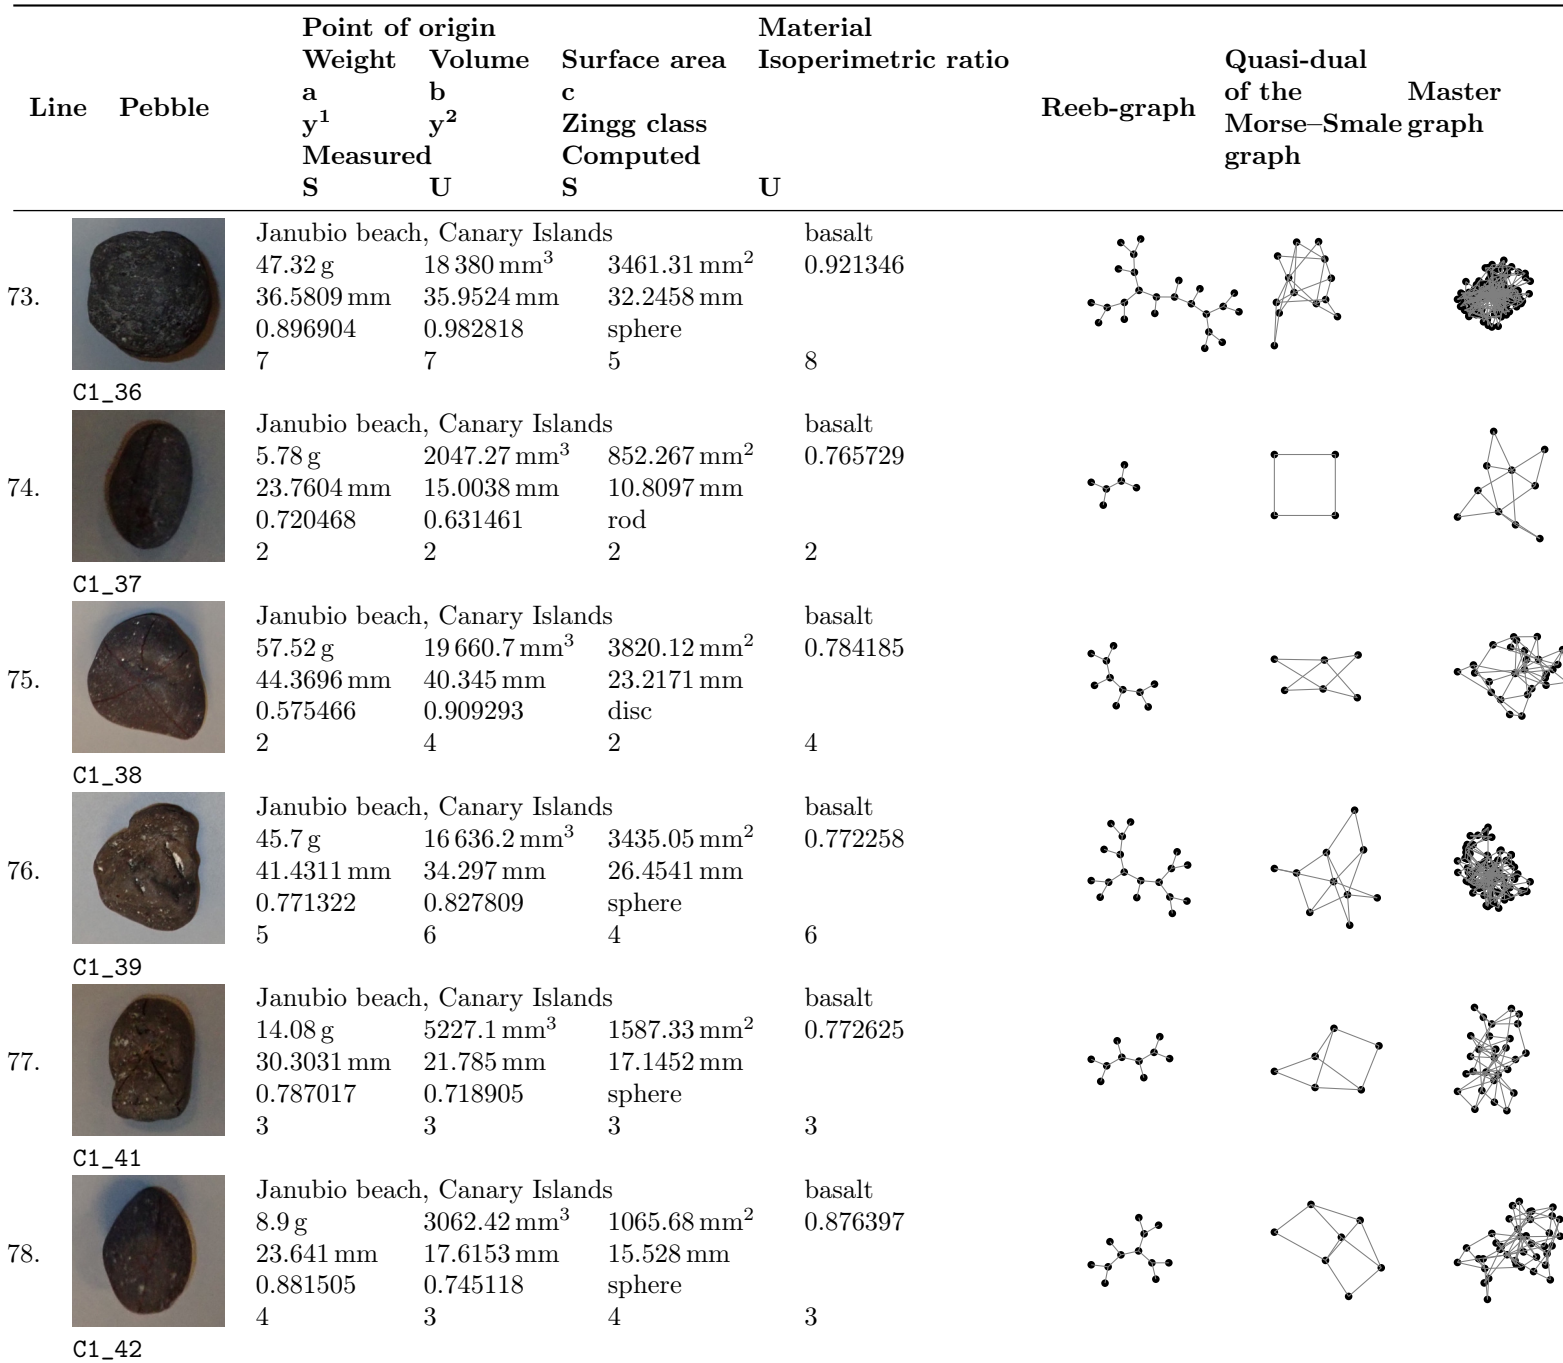  | 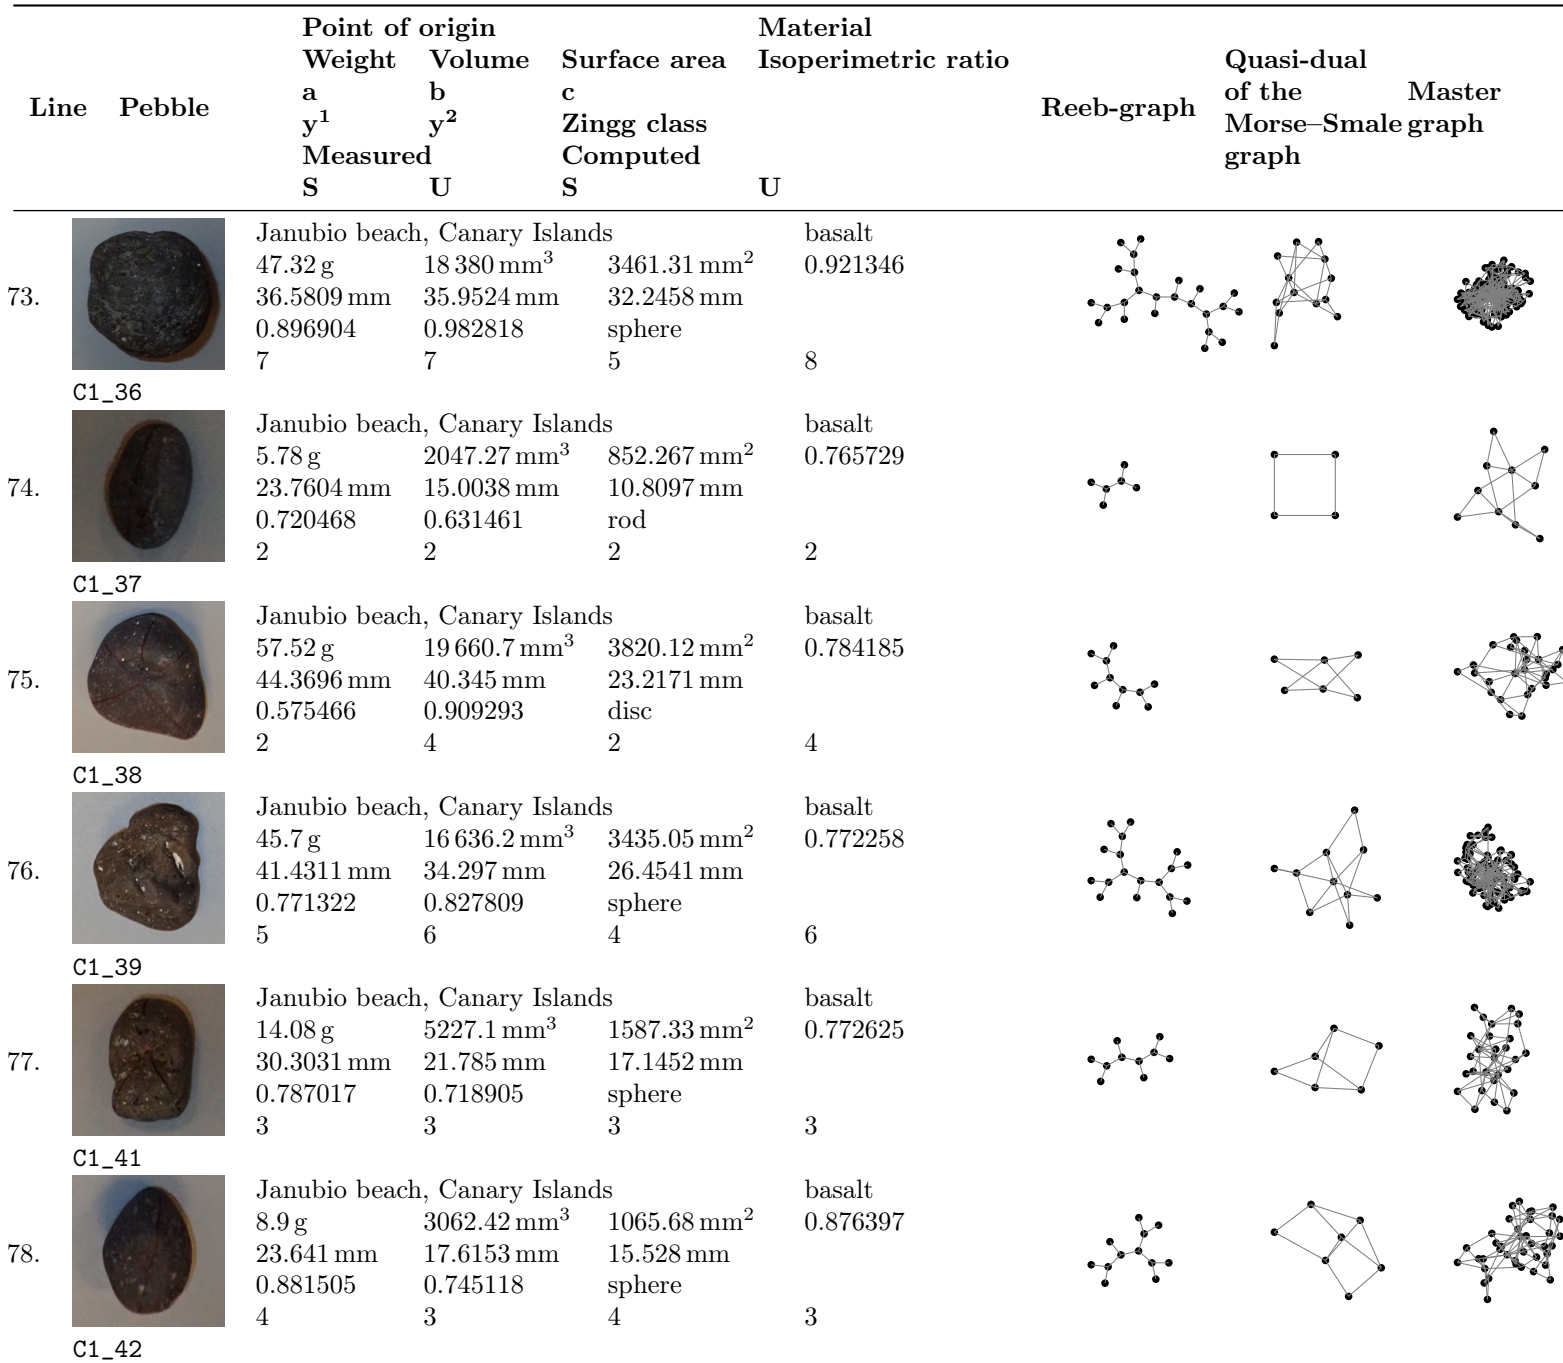  |
|      |                                                                                     | 45.7 g                        | 16 636.2 mm <sup>3</sup> | 3435.05 mm <sup>2</sup> | 0.772258            |                                                                                       |                                                                                       |                                                                                       |
|      |                                                                                     | 41.4311 mm                    | 34.297 mm                | 26.4541 mm              |                     |                                                                                       |                                                                                       |                                                                                       |
|      |                                                                                     | 0.771322                      | 0.827809                 | sphere                  |                     |                                                                                       |                                                                                       |                                                                                       |
|      |                                                                                     | 5                             | 6                        | 4                       | 6                   |                                                                                       |                                                                                       |                                                                                       |
|      |                                                                                     | C1_39                         |                          |                         |                     |                                                                                       |                                                                                       |                                                                                       |
| 77.  | 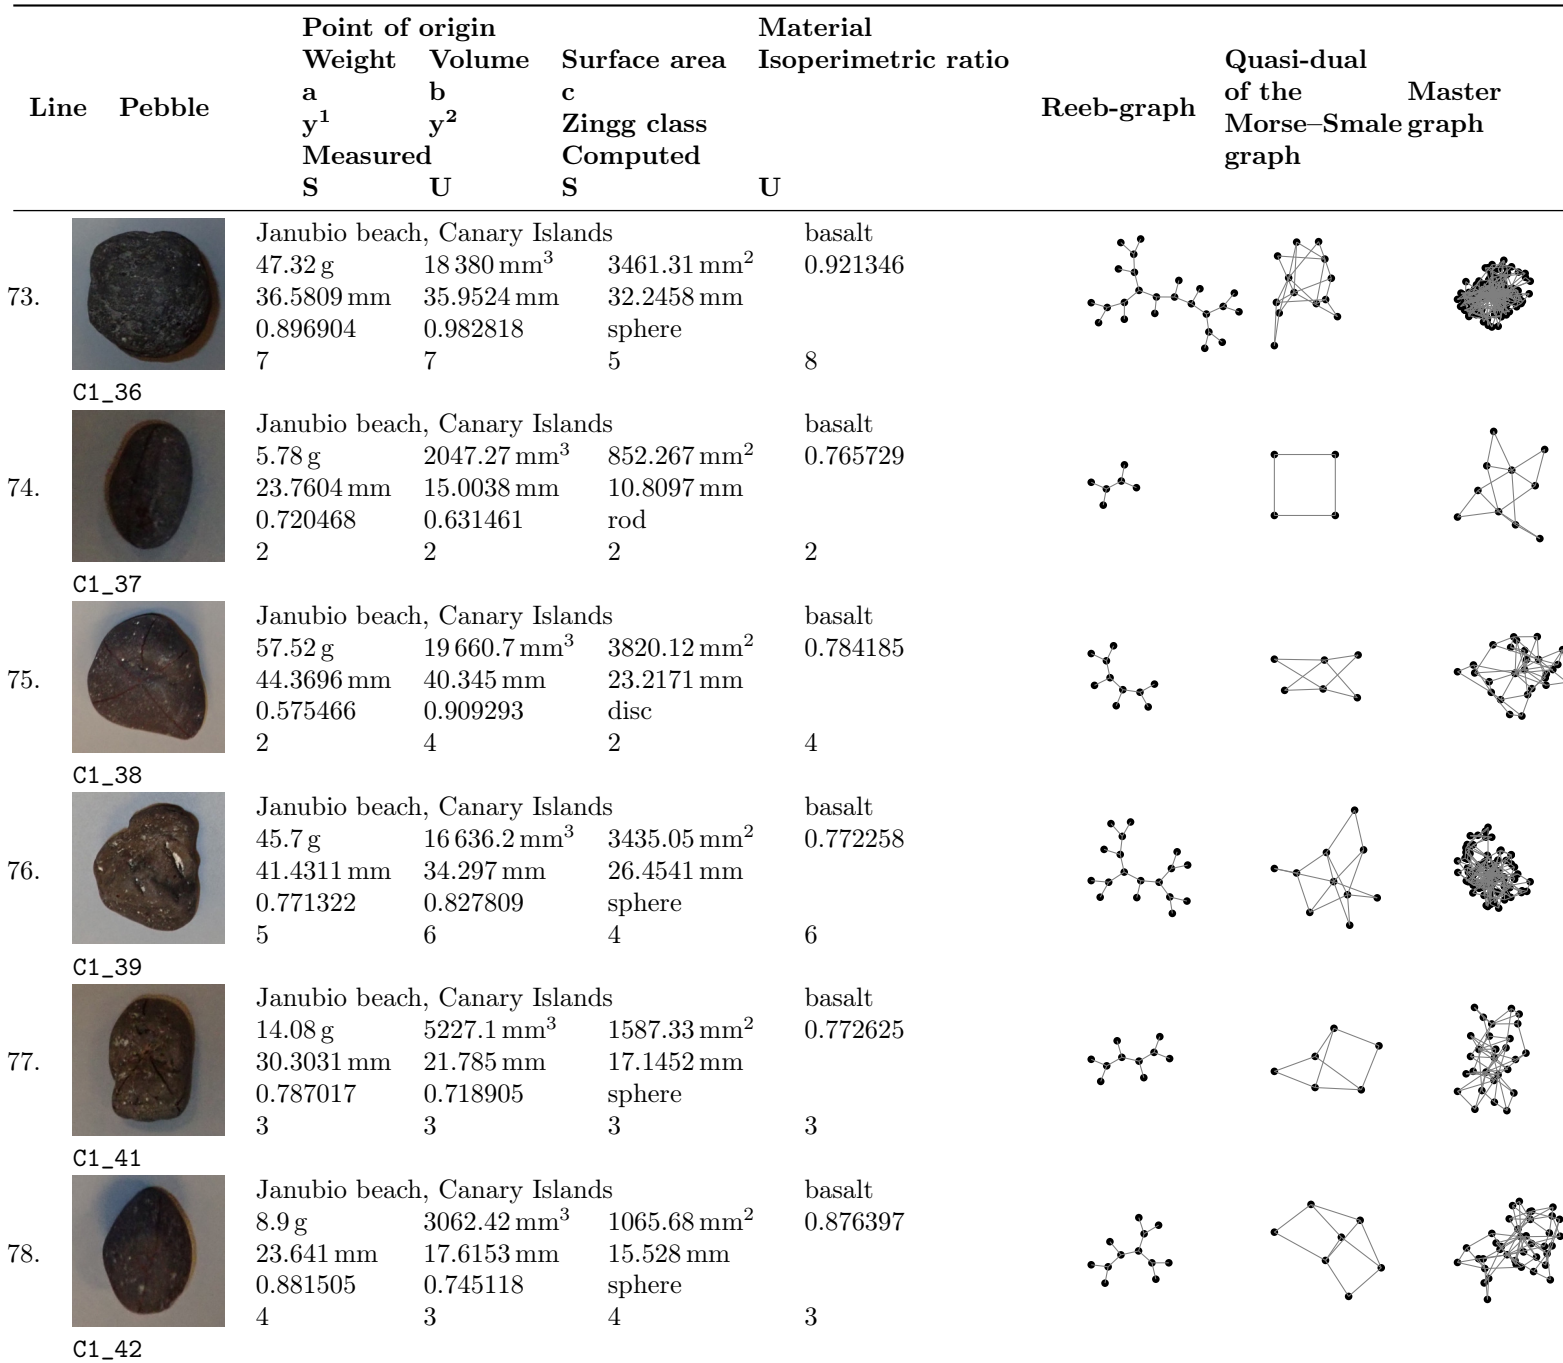 | Janubio beach, Canary Islands |                          |                         | basalt              | 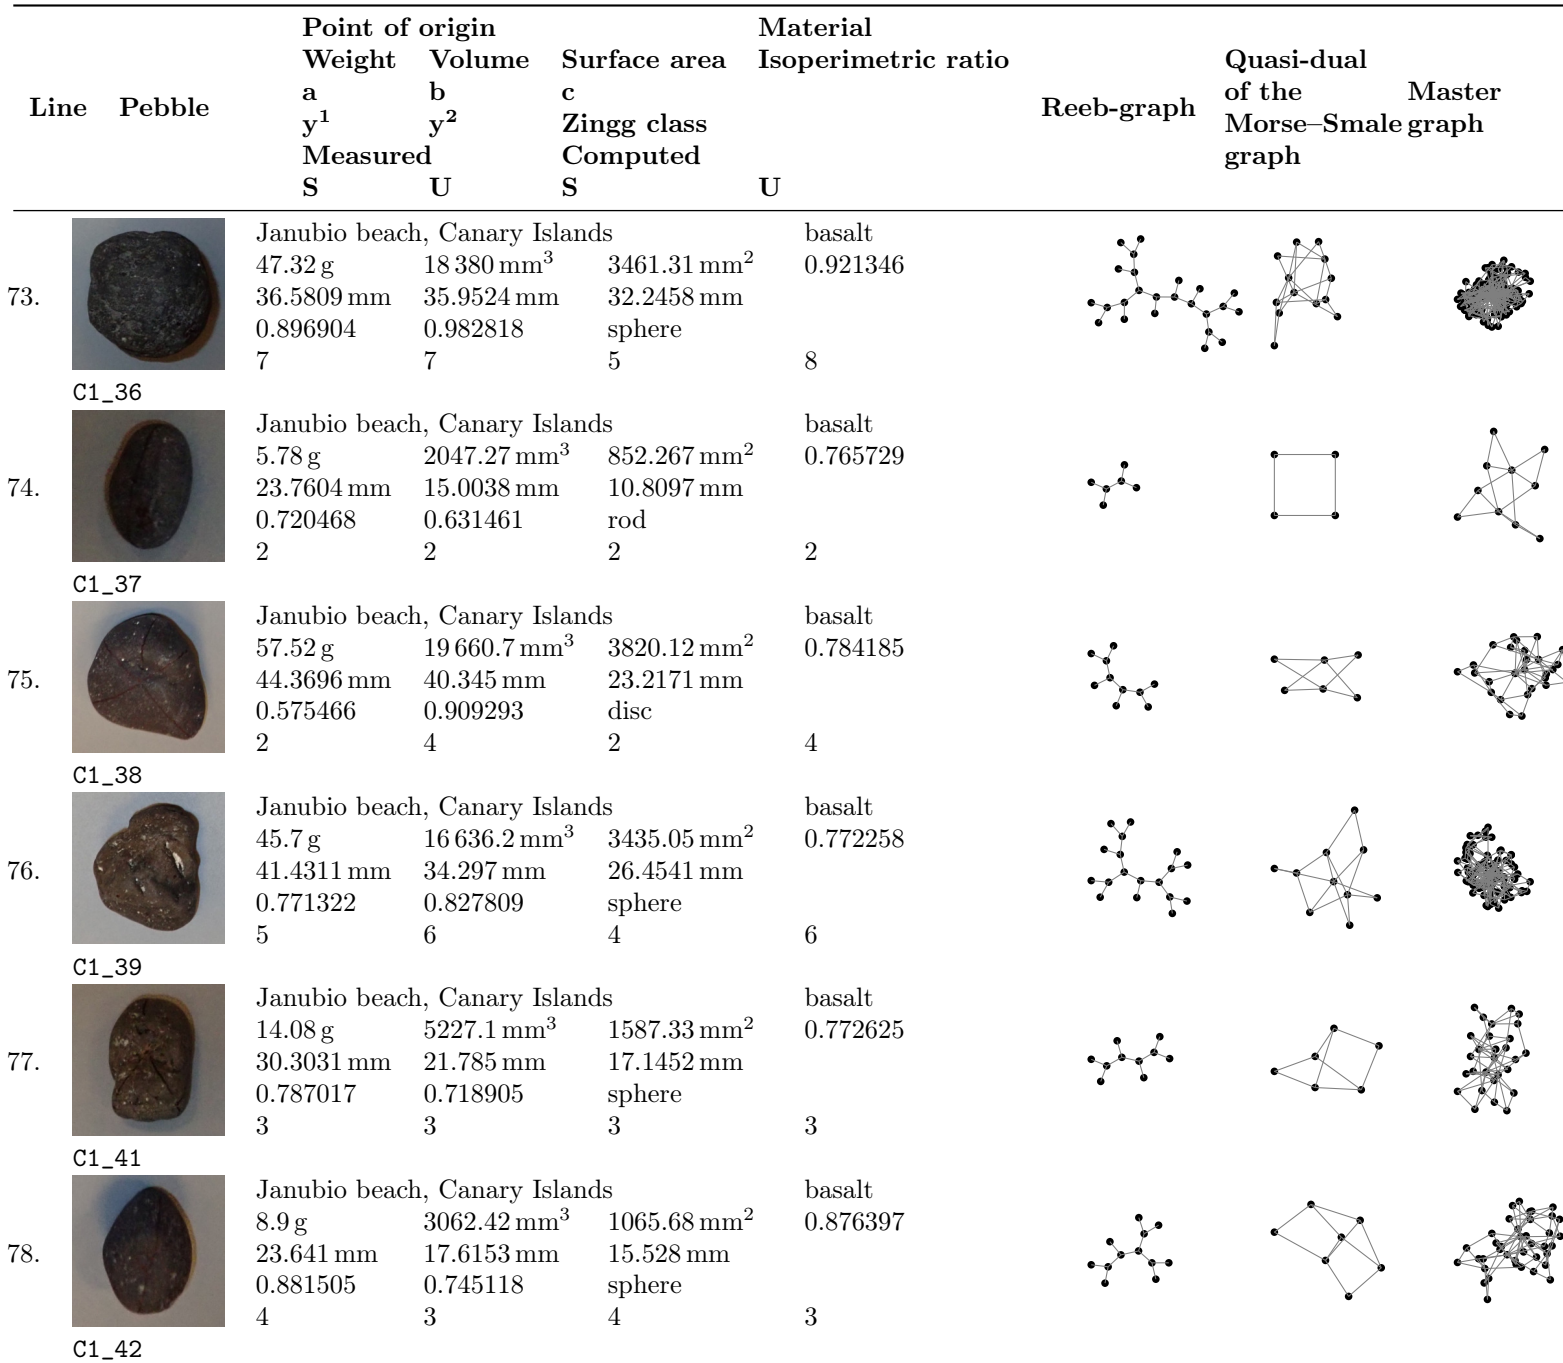 | 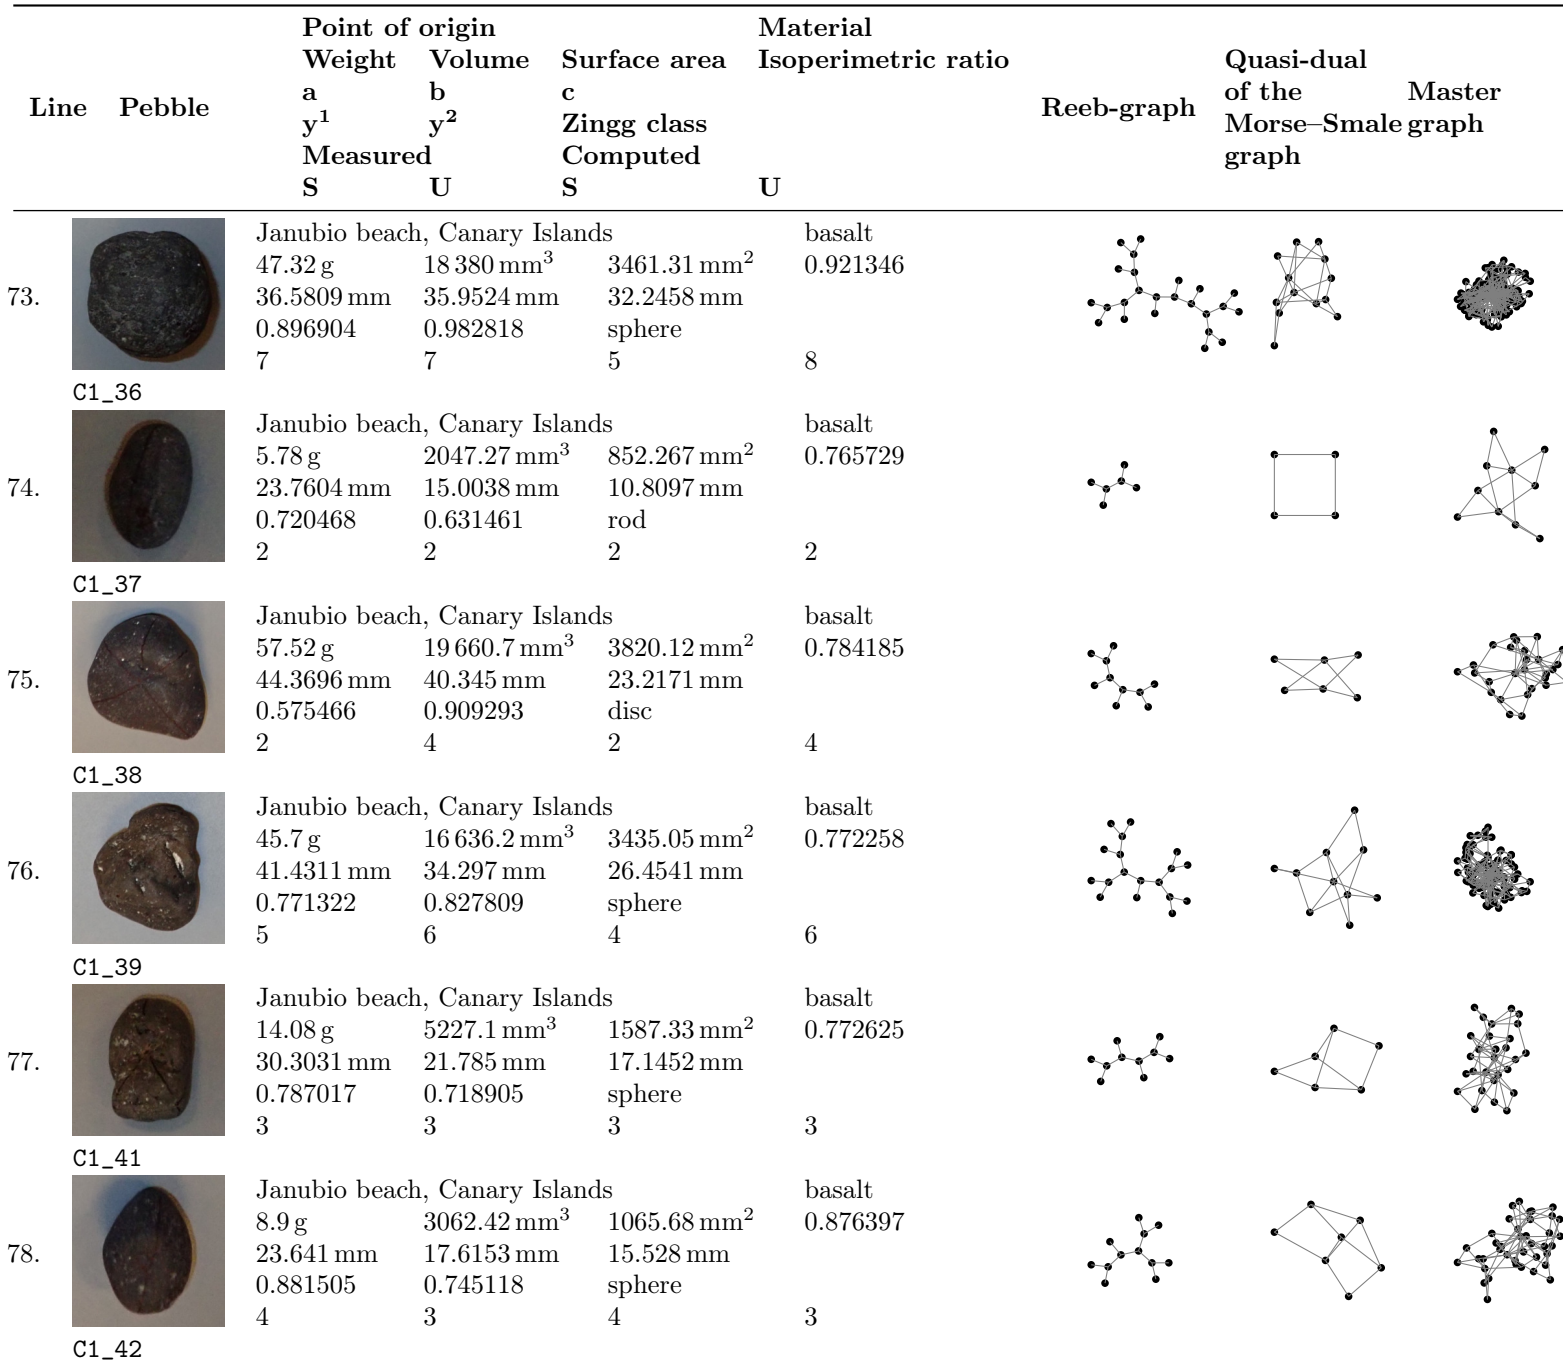 | 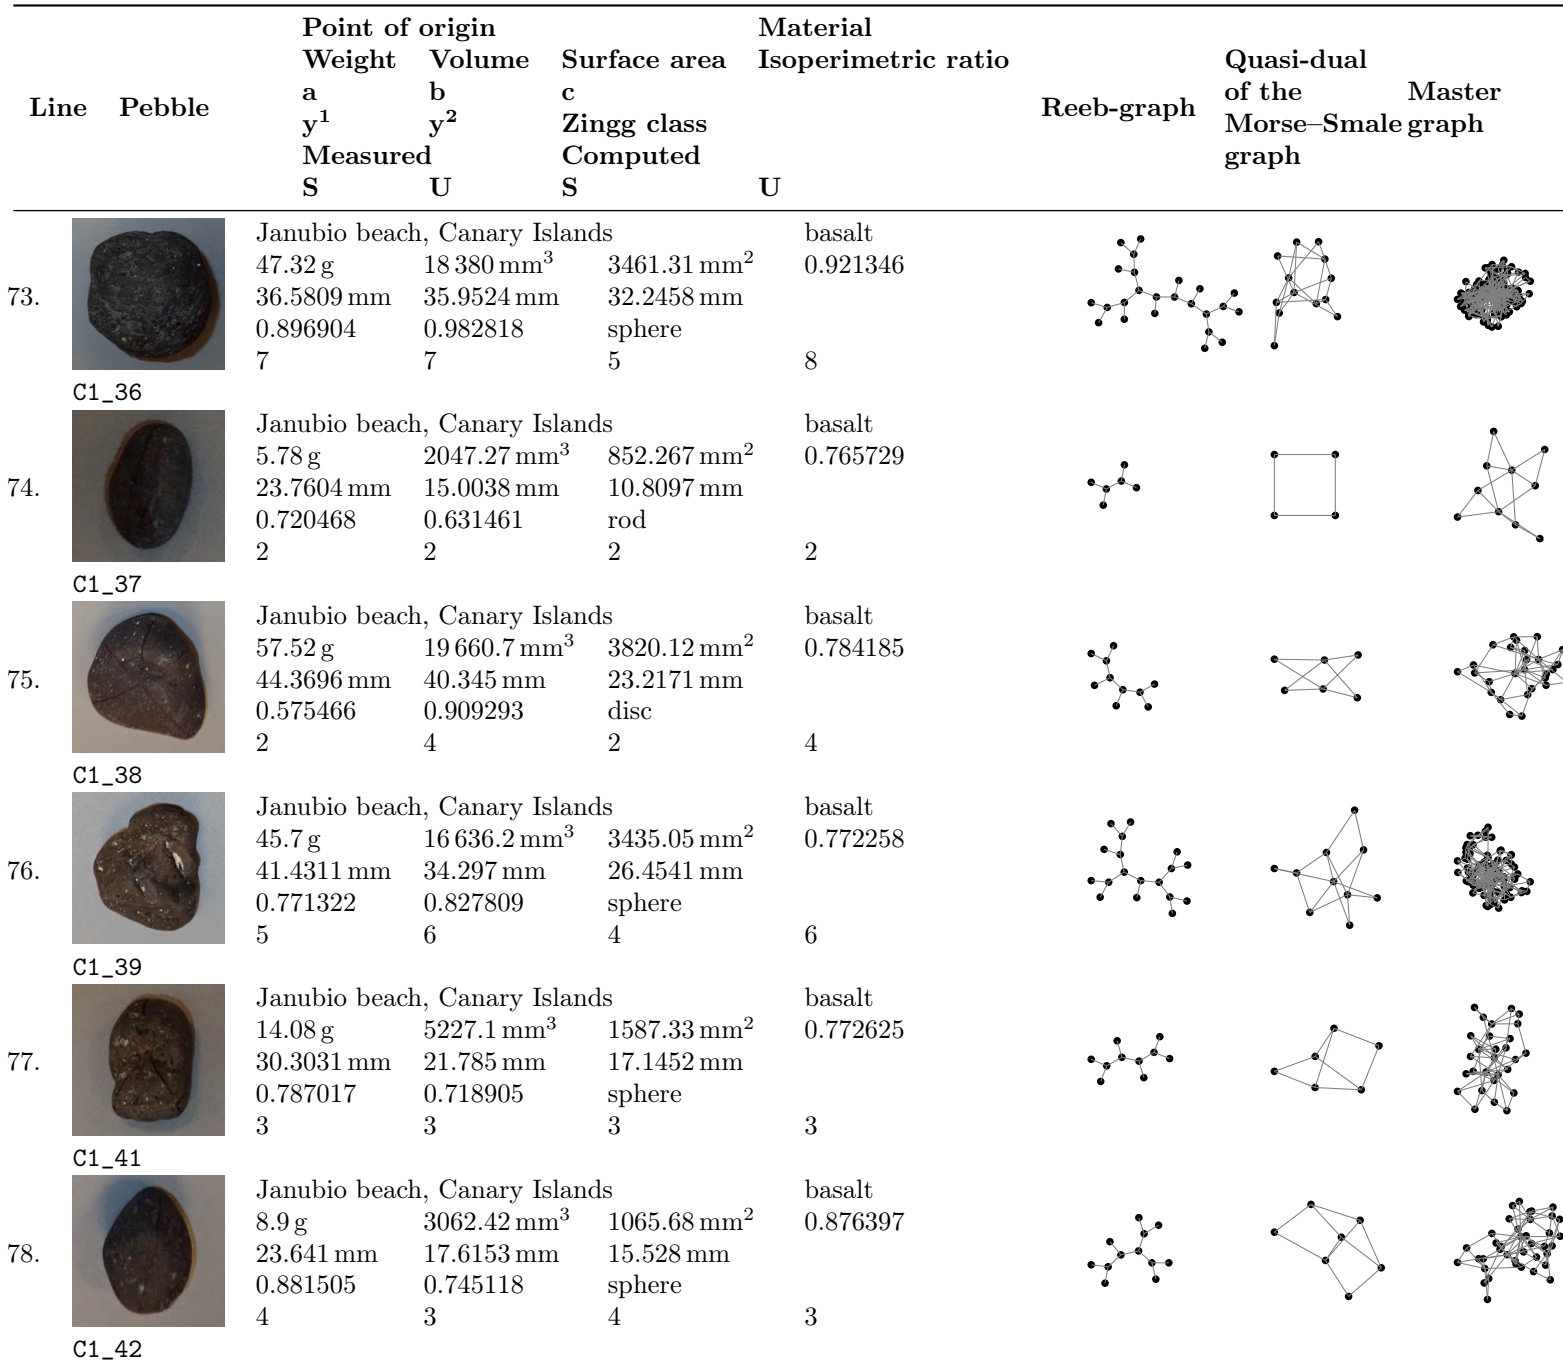 |
|      |                                                                                     | 14.08 g                       | 5227.1 mm <sup>3</sup>   | 1587.33 mm <sup>2</sup> | 0.772625            |                                                                                       |                                                                                       |                                                                                       |
|      |                                                                                     | 30.3031 mm                    | 21.785 mm                | 17.1452 mm              |                     |                                                                                       |                                                                                       |                                                                                       |
|      |                                                                                     | 0.787017                      | 0.718905                 | sphere                  |                     |                                                                                       |                                                                                       |                                                                                       |
|      |                                                                                     | 3                             | 3                        | 3                       | 3                   |                                                                                       |                                                                                       |                                                                                       |
|      |                                                                                     | C1_41                         |                          |                         |                     |                                                                                       |                                                                                       |                                                                                       |
| 78.  | 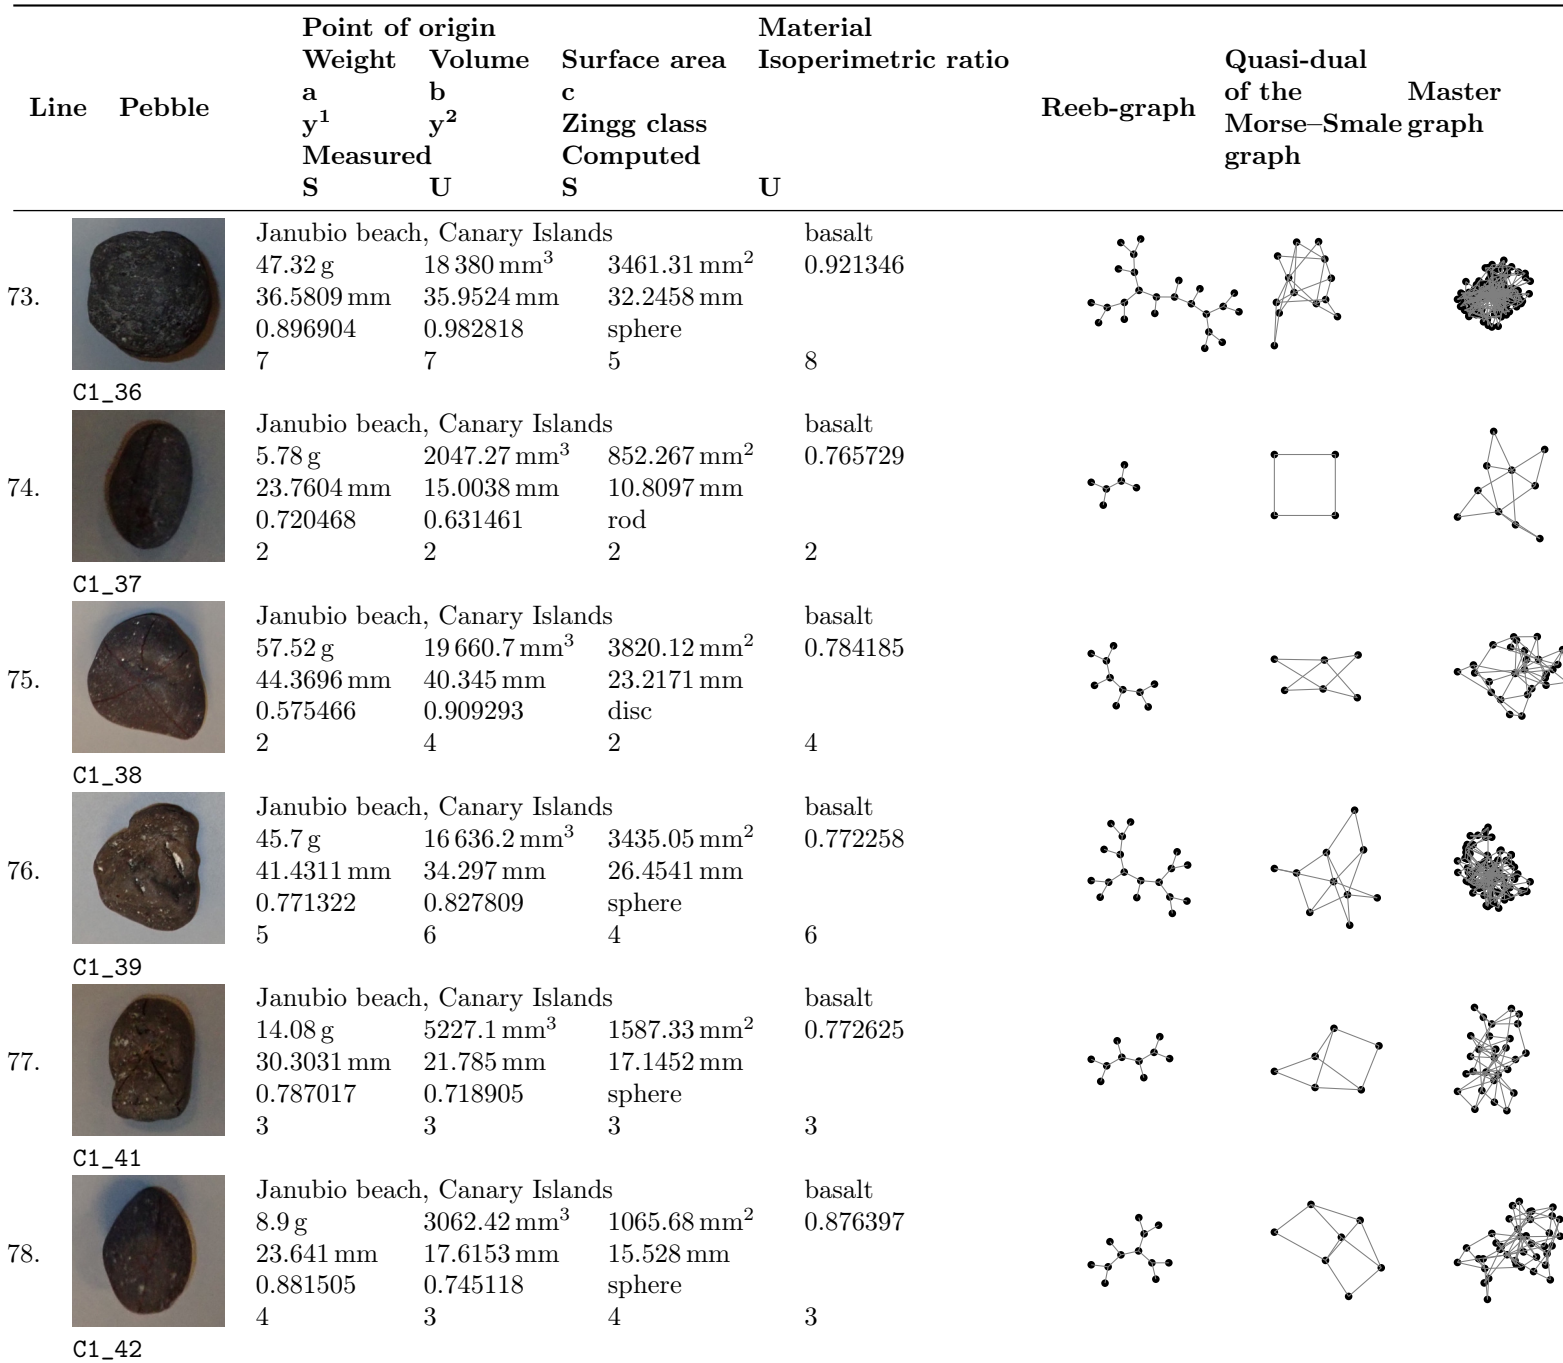 | Janubio beach, Canary Islands |                          |                         | basalt              | 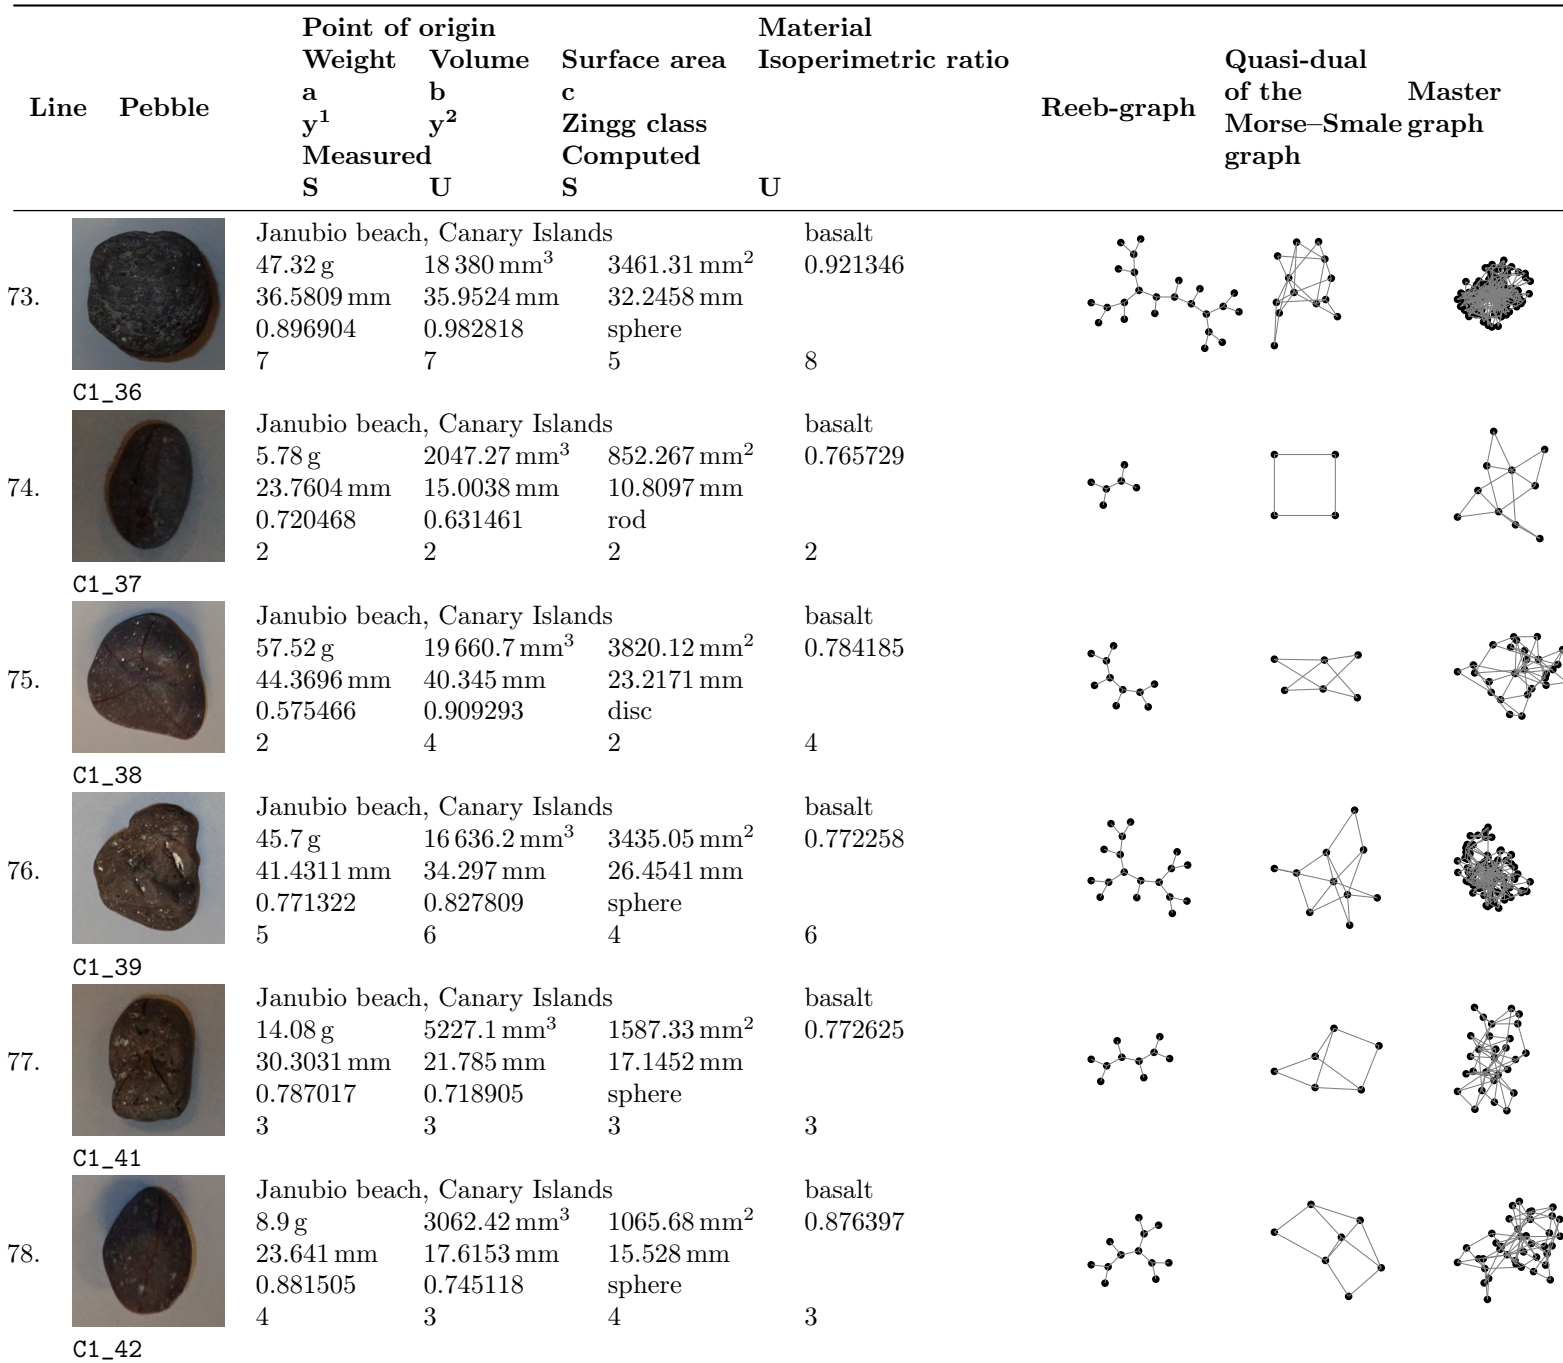 | 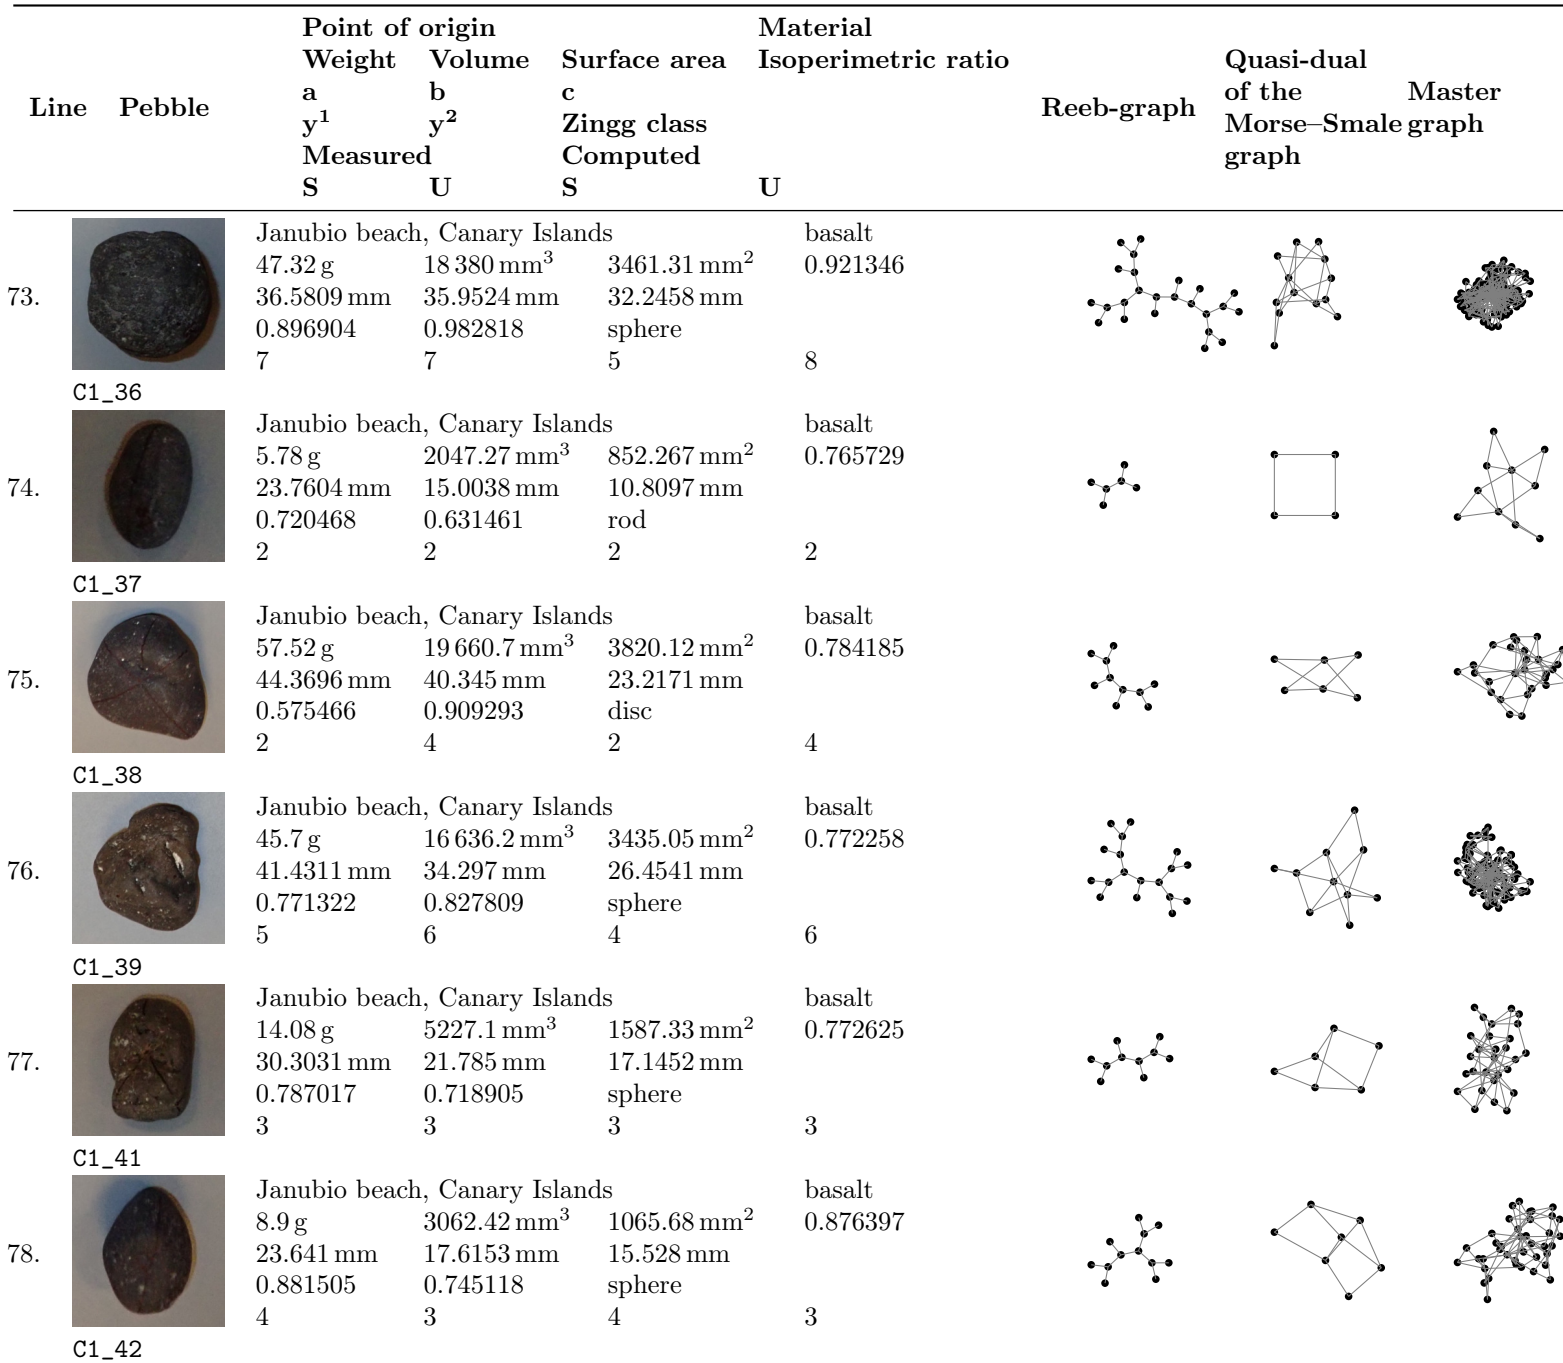 | 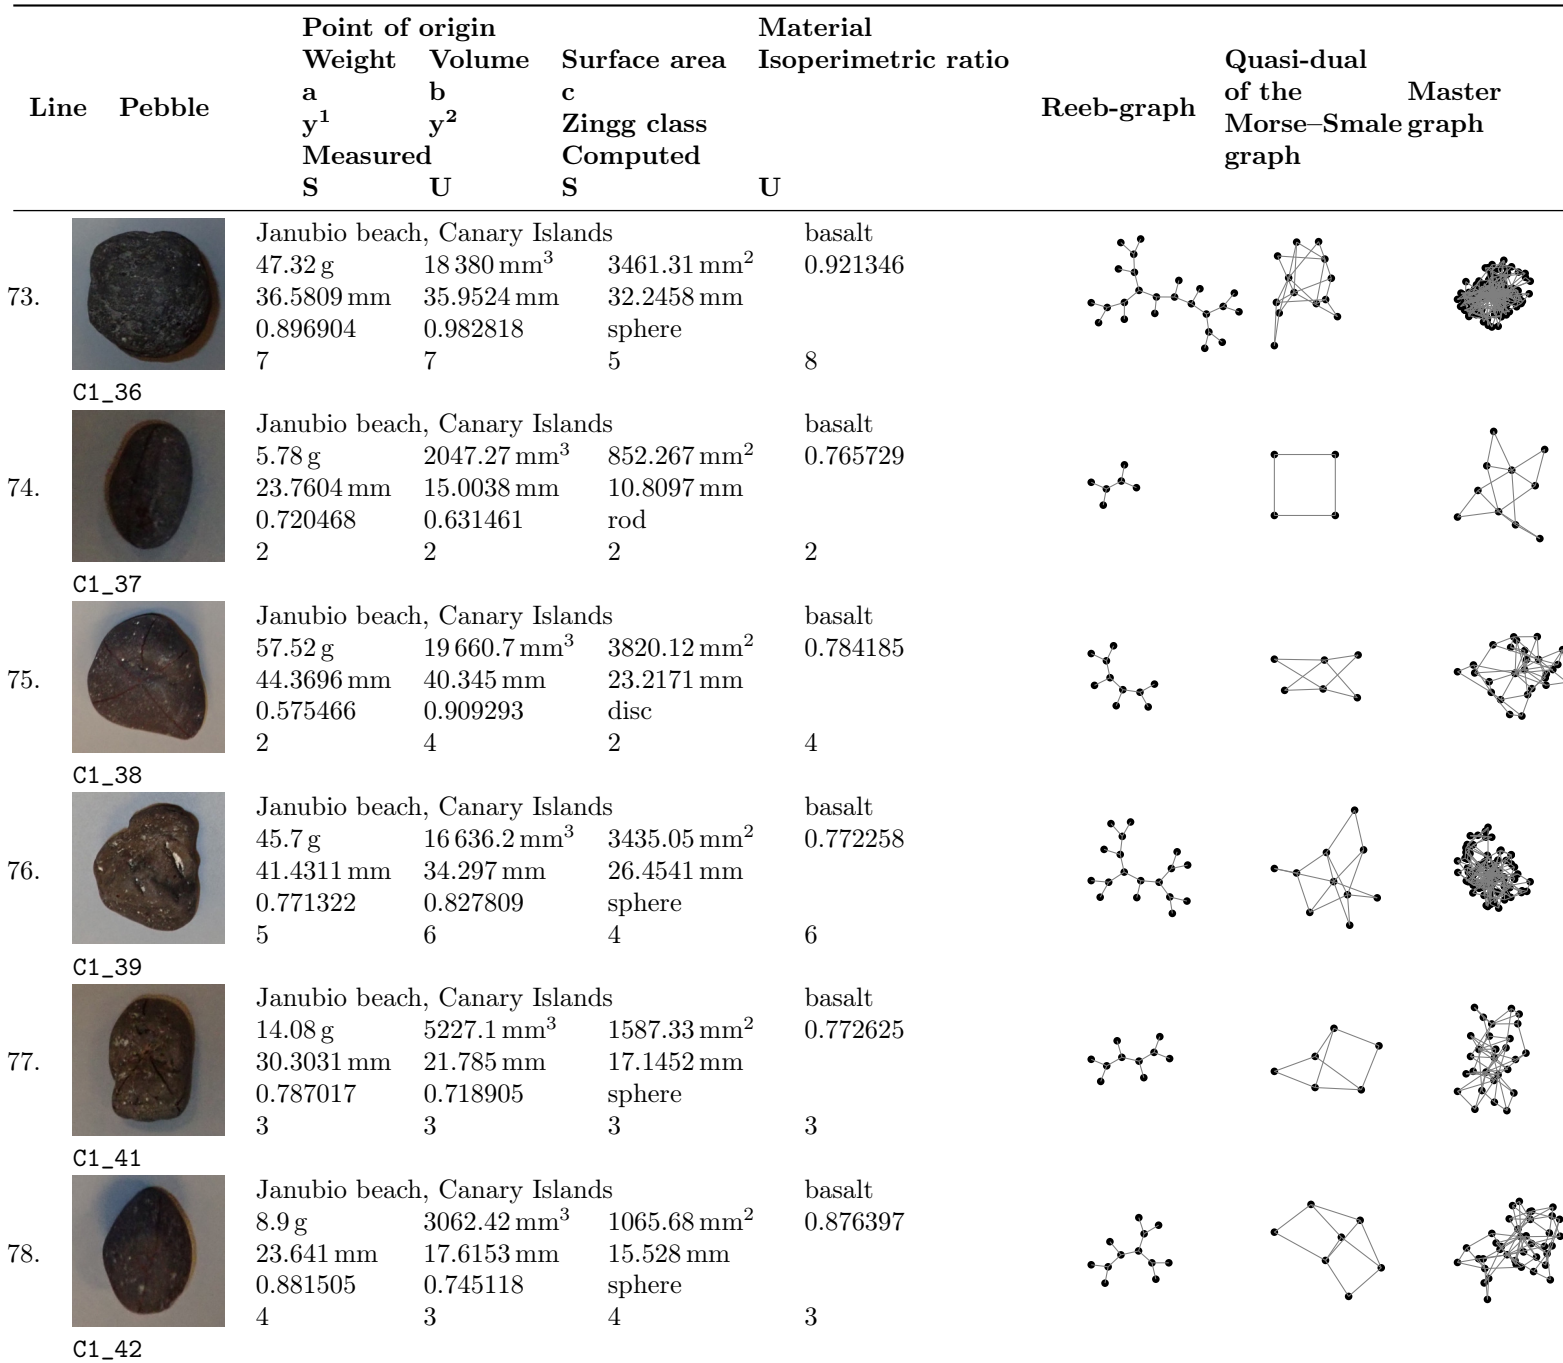 |
|      |                                                                                     | 8.9 g                         | 3062.42 mm <sup>3</sup>  | 1065.68 mm <sup>2</sup> | 0.876397            |                                                                                       |                                                                                       |                                                                                       |
|      |                                                                                     | 23.641 mm                     | 17.6153 mm               | 15.528 mm               |                     |                                                                                       |                                                                                       |                                                                                       |
|      |                                                                                     | 0.881505                      | 0.745118                 | sphere                  |                     |                                                                                       |                                                                                       |                                                                                       |
|      |                                                                                     | 4                             | 3                        | 4                       | 3                   |                                                                                       |                                                                                       |                                                                                       |
|      |                                                                                     | C1_42                         |                          |                         |                     |                                                                                       |                                                                                       |                                                                                       |

| Line | Pebble                                                                              | Point of origin                 |                          |                              | Material | Isoperimetric ratio | Reeb-graph                                                                            | Quasi-dual<br>of the<br>Morse–Smale<br>graph                                          | Master<br>graph                                                                       |
|------|-------------------------------------------------------------------------------------|---------------------------------|--------------------------|------------------------------|----------|---------------------|---------------------------------------------------------------------------------------|---------------------------------------------------------------------------------------|---------------------------------------------------------------------------------------|
|      |                                                                                     | Weight                          | Volume                   | Surface area                 |          |                     |                                                                                       |                                                                                       |                                                                                       |
|      |                                                                                     | a                               | b                        | c                            |          |                     |                                                                                       |                                                                                       |                                                                                       |
|      |                                                                                     | y <sup>1</sup><br>Measured<br>S | y <sup>2</sup><br>U      | Zingg class<br>Computed<br>S |          |                     |                                                                                       |                                                                                       |                                                                                       |
|      |                                                                                     |                                 |                          |                              | U        |                     |                                                                                       |                                                                                       |                                                                                       |
| 79.  | 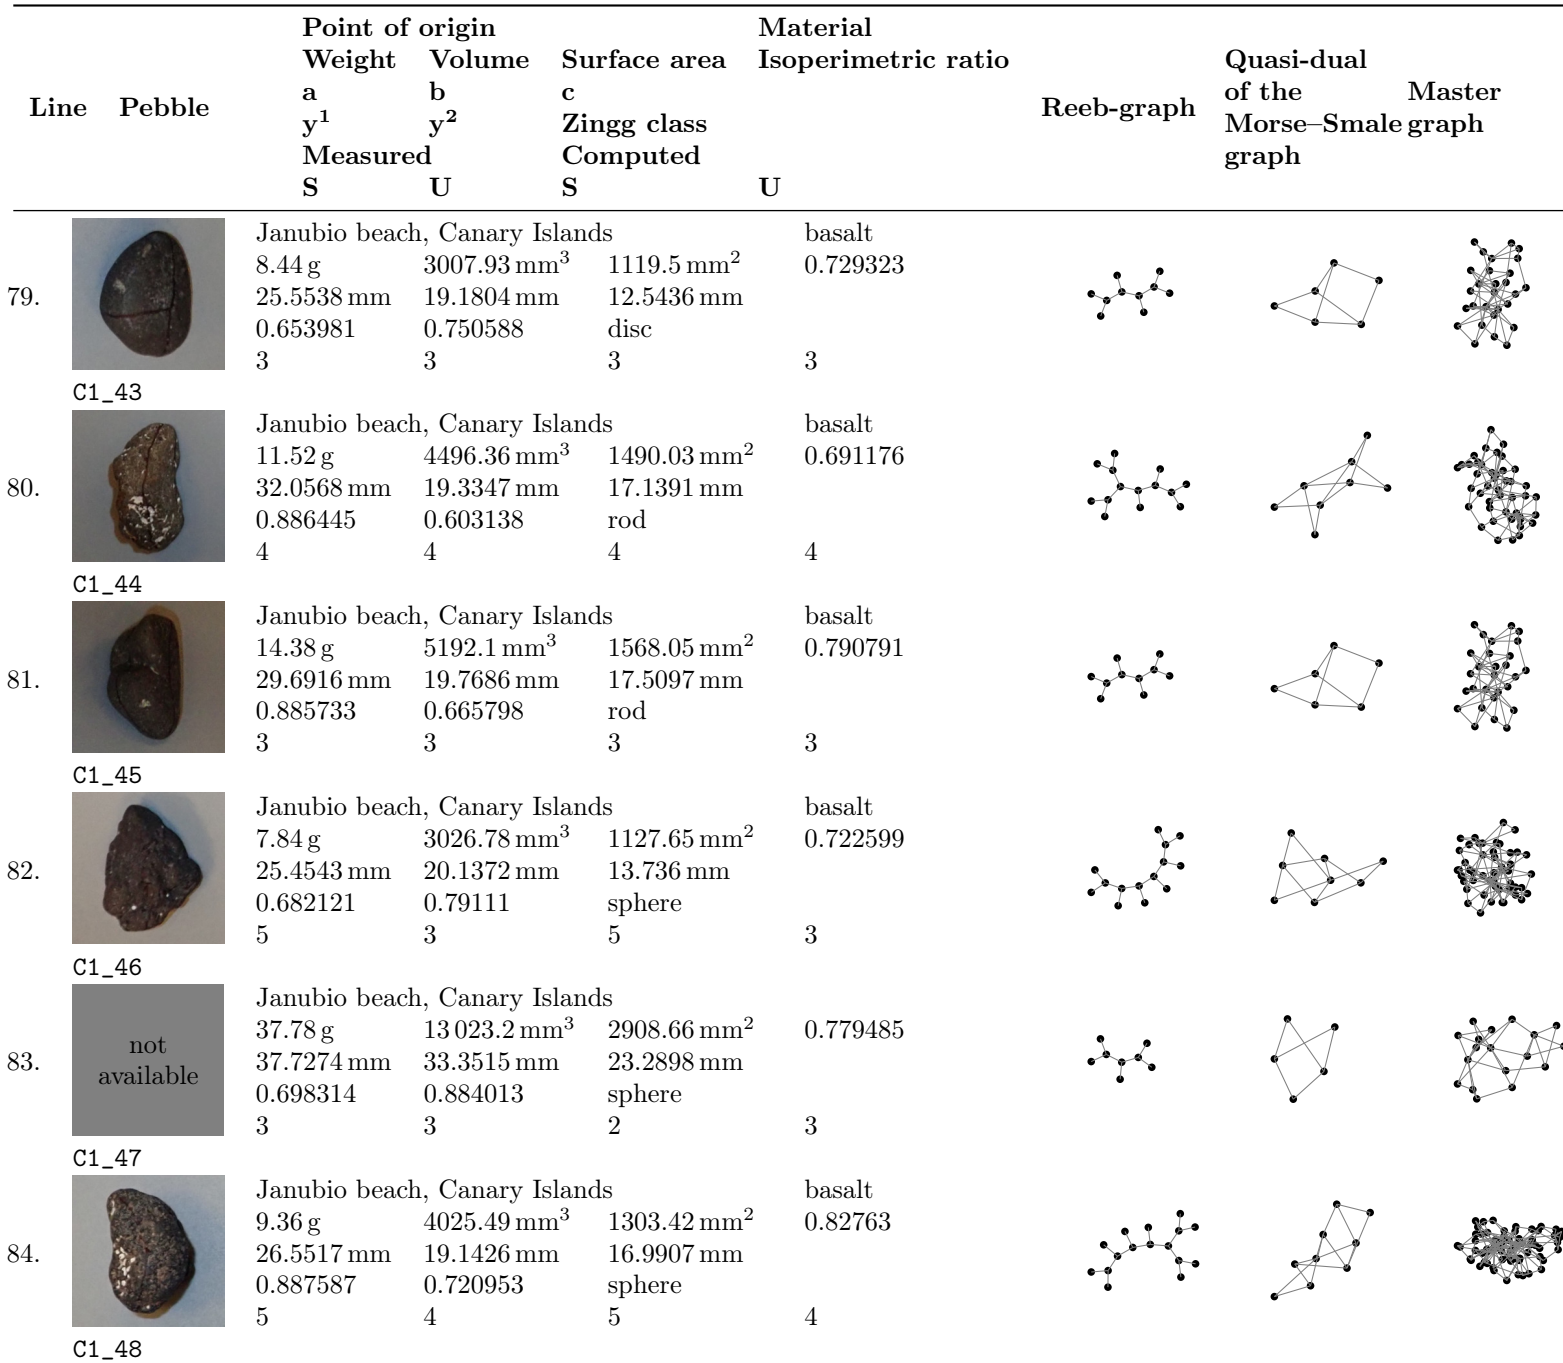   | Janubio beach, Canary Islands   |                          |                              | basalt   | 0.729323            | 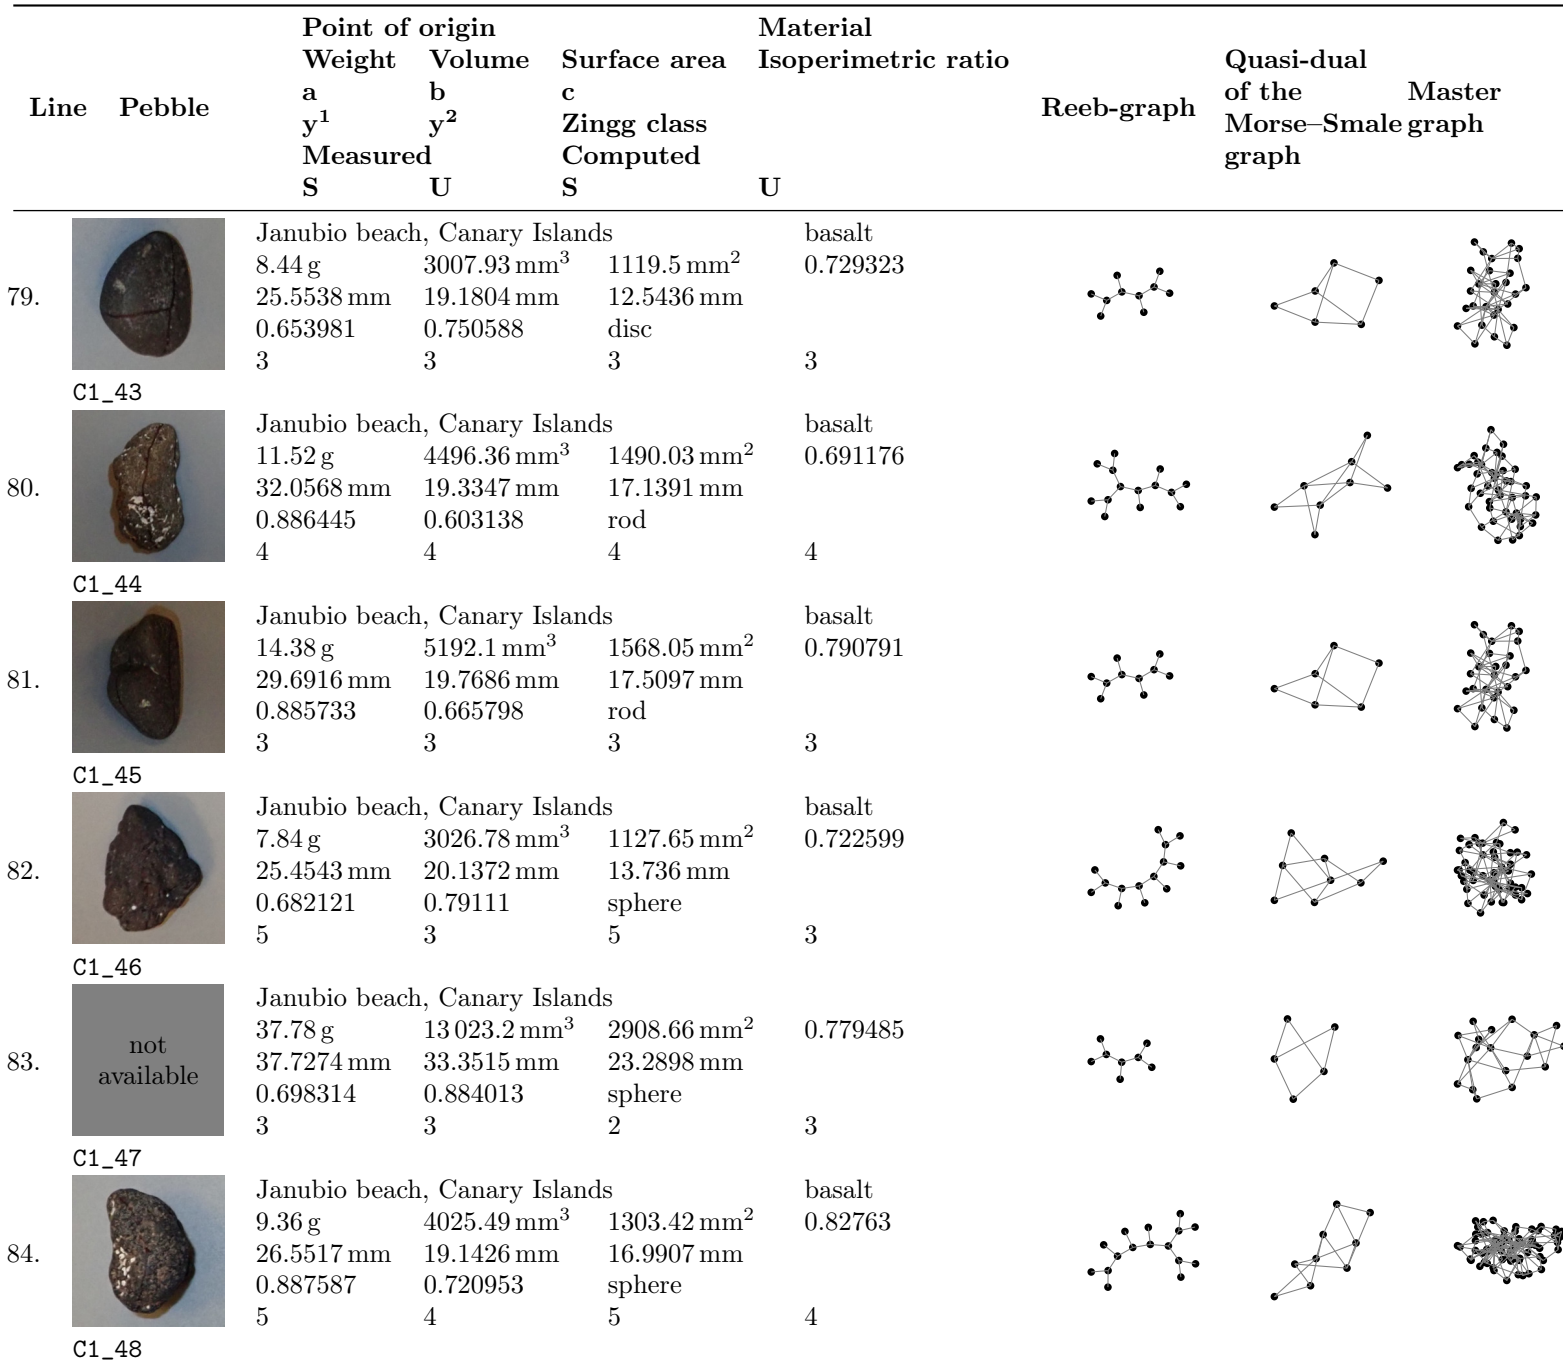   | 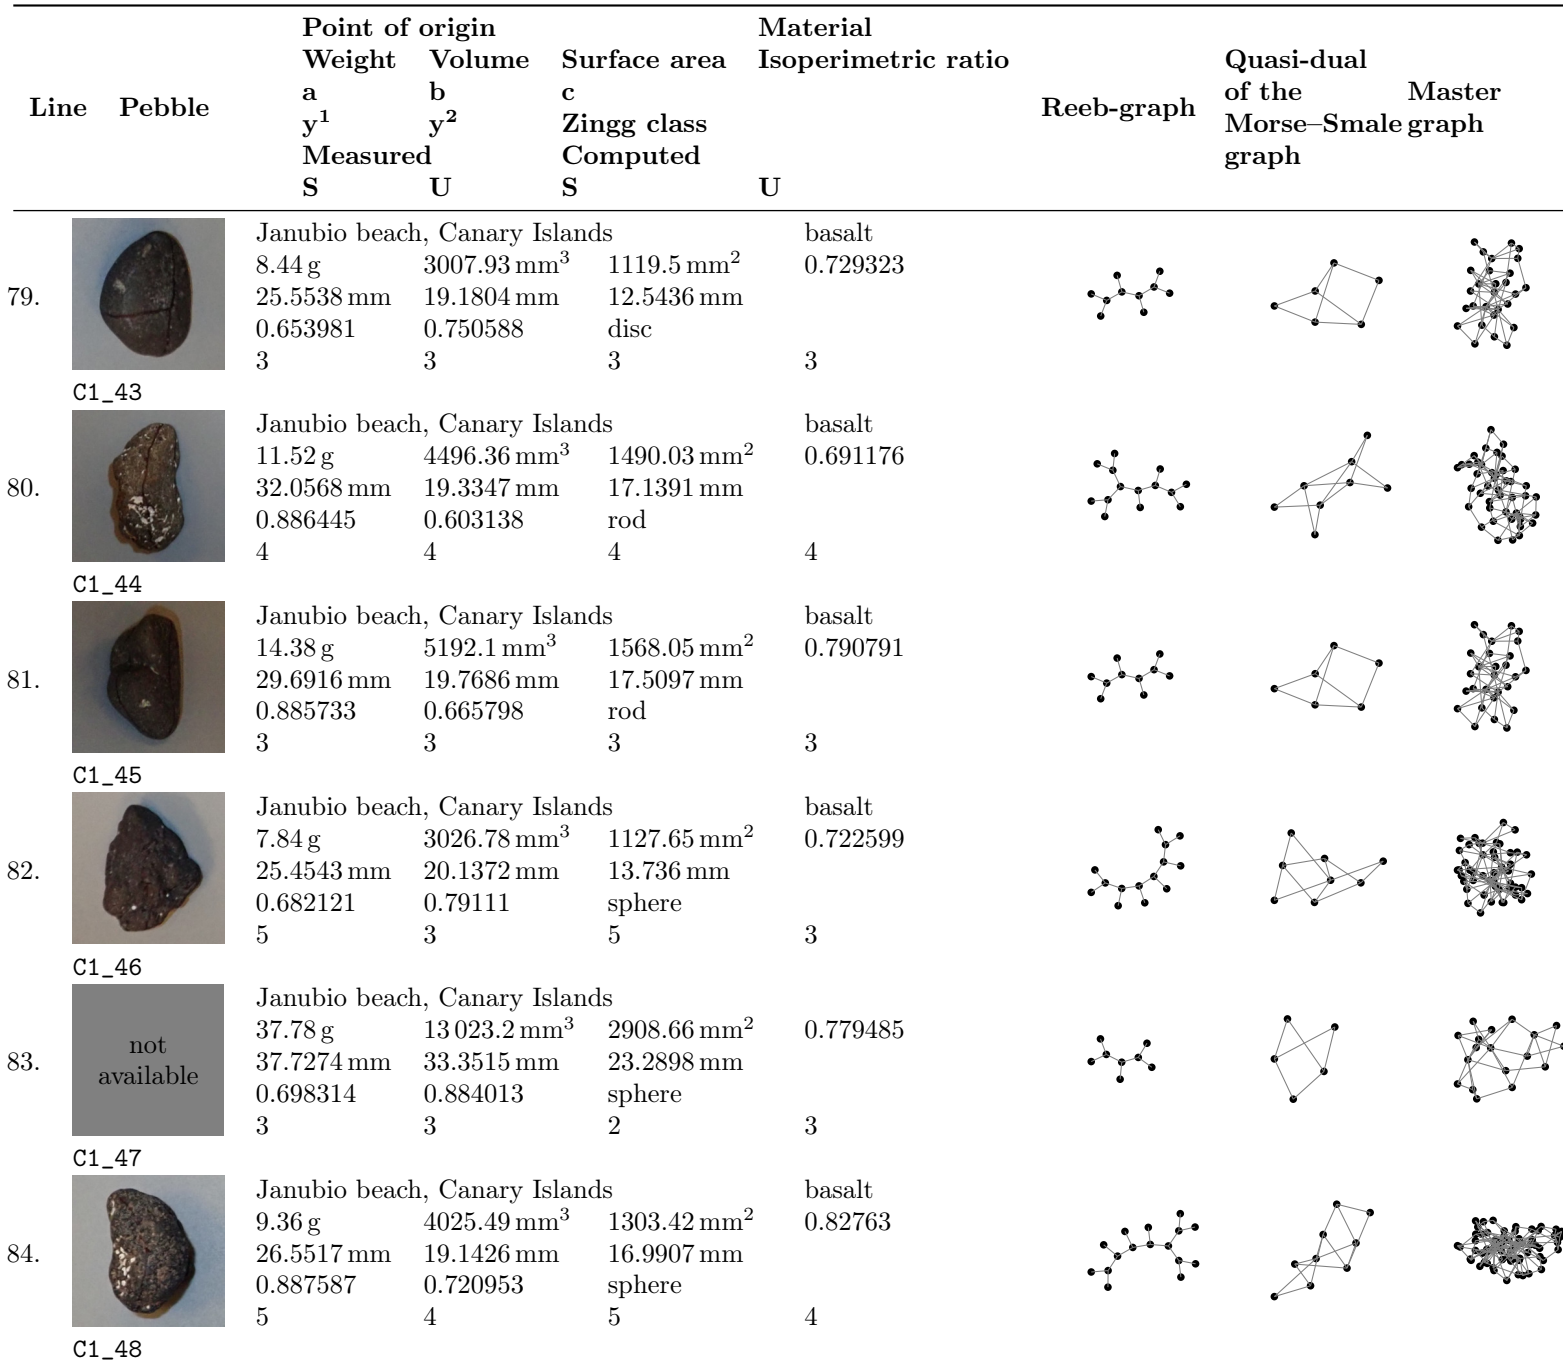   | 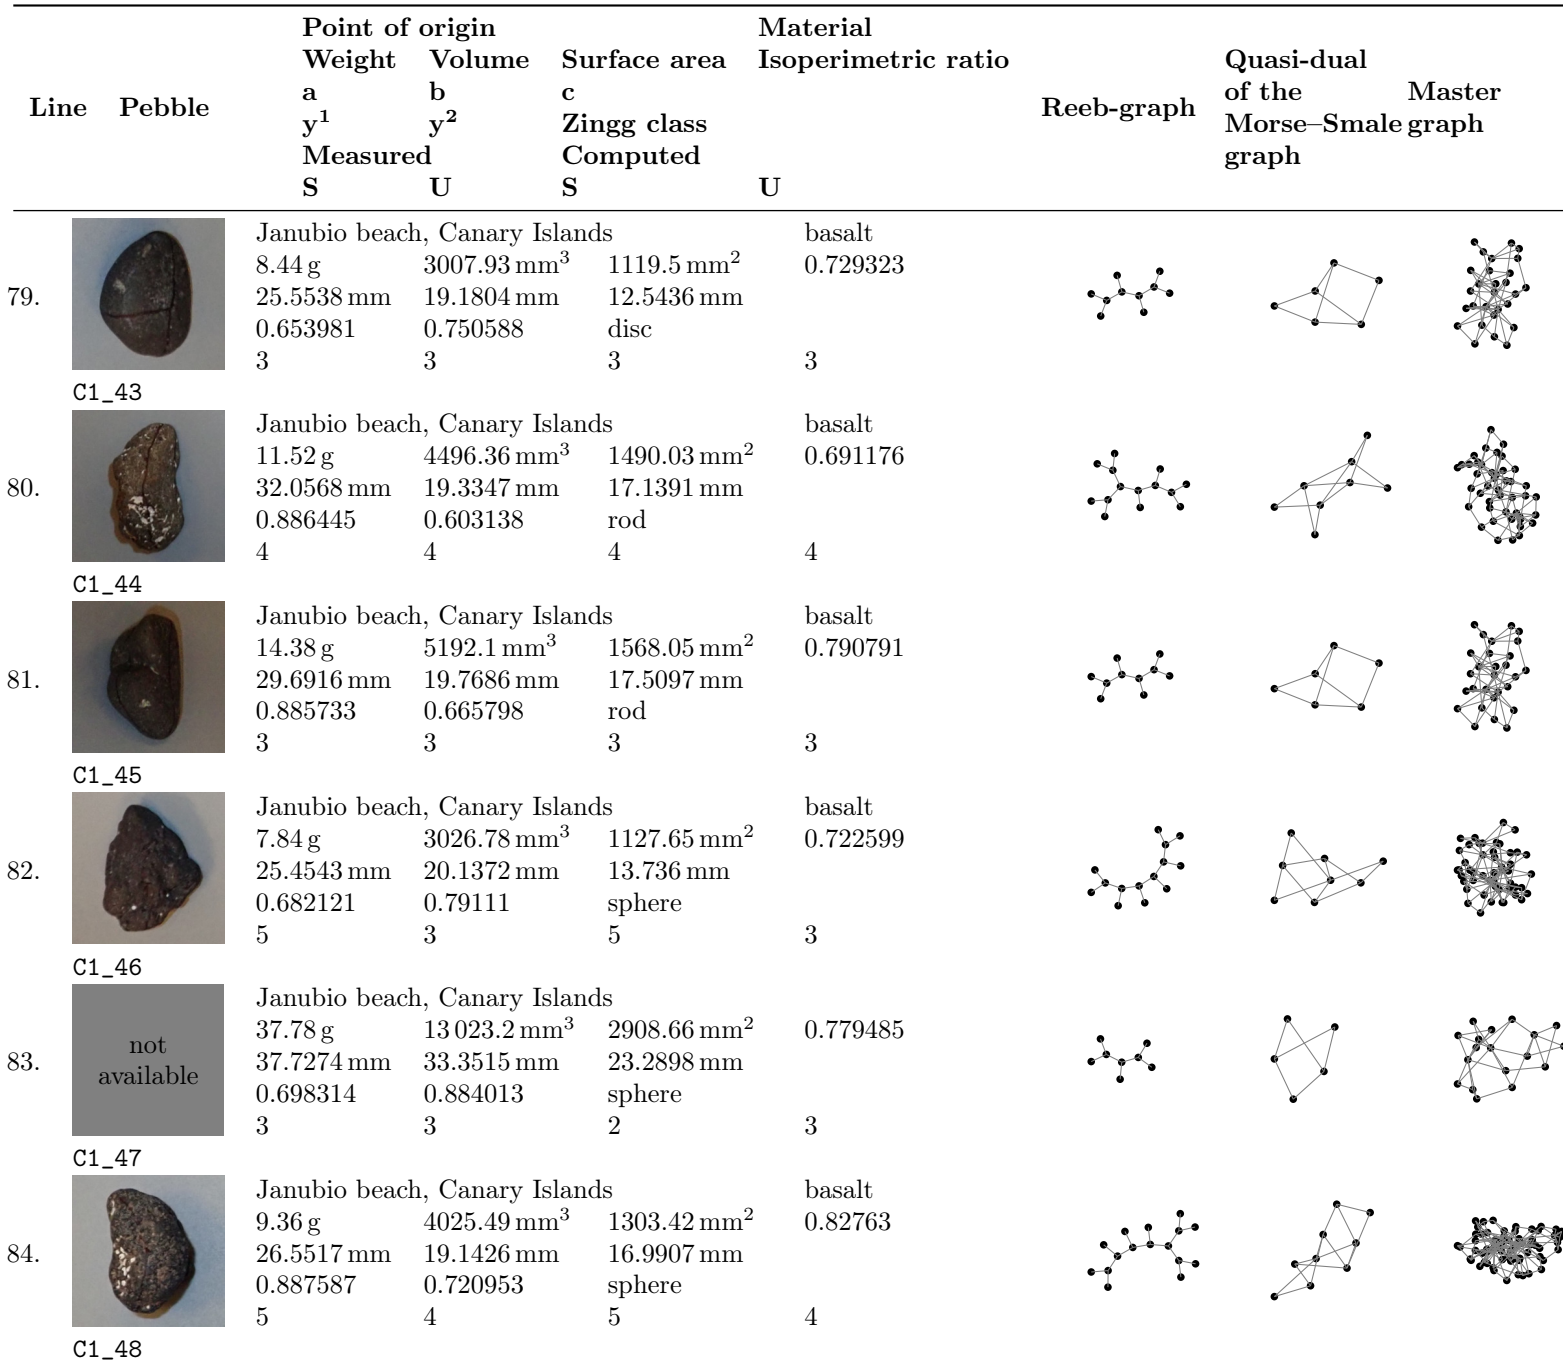   |
|      |                                                                                     | 8.44 g                          | 3007.93 mm <sup>3</sup>  | 1119.5 mm <sup>2</sup>       |          |                     |                                                                                       |                                                                                       |                                                                                       |
|      |                                                                                     | 25.5538 mm                      | 19.1804 mm               | 12.5436 mm                   |          |                     |                                                                                       |                                                                                       |                                                                                       |
|      |                                                                                     | 0.653981                        | 0.750588                 | disc                         |          |                     |                                                                                       |                                                                                       |                                                                                       |
|      |                                                                                     | 3                               | 3                        | 3                            |          |                     |                                                                                       |                                                                                       |                                                                                       |
|      | C1_43                                                                               |                                 |                          |                              |          |                     |                                                                                       |                                                                                       |                                                                                       |
| 80.  | 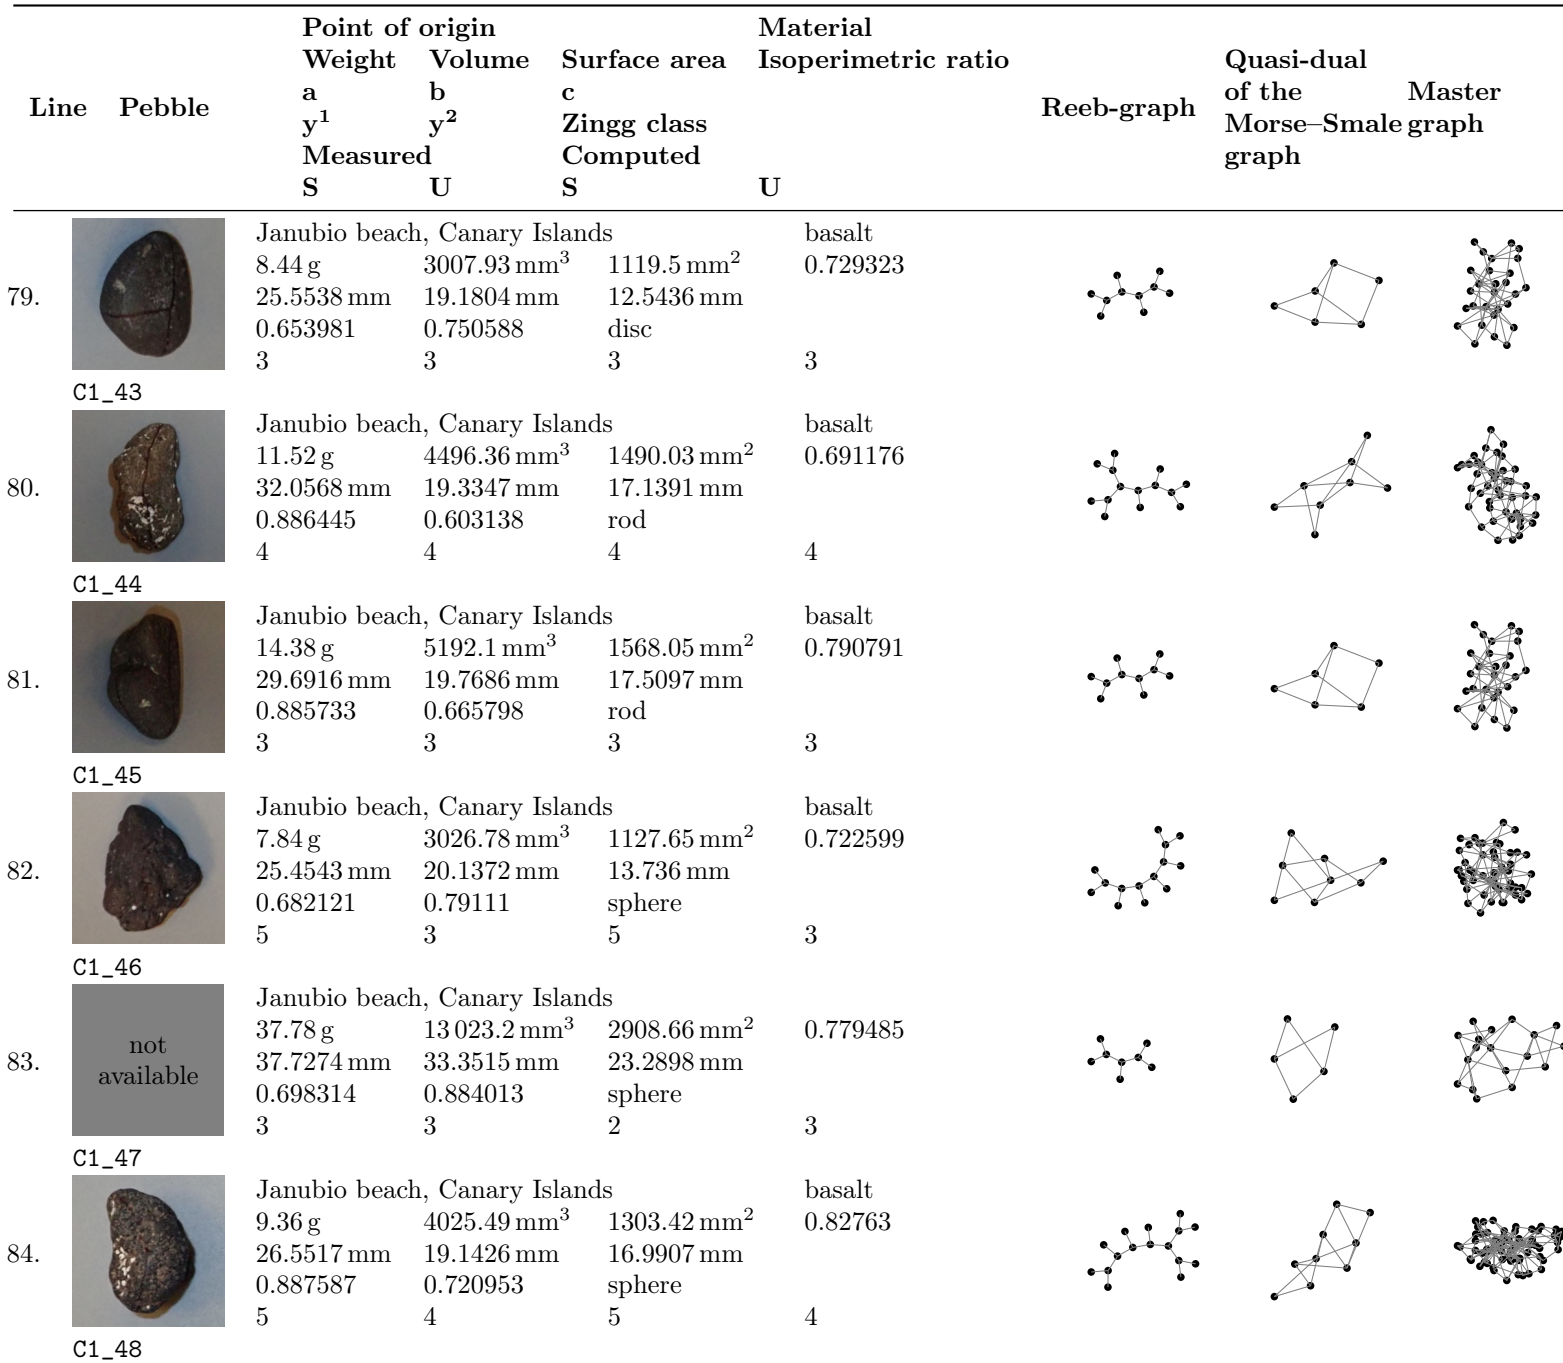   | Janubio beach, Canary Islands   |                          |                              | basalt   | 0.691176            | 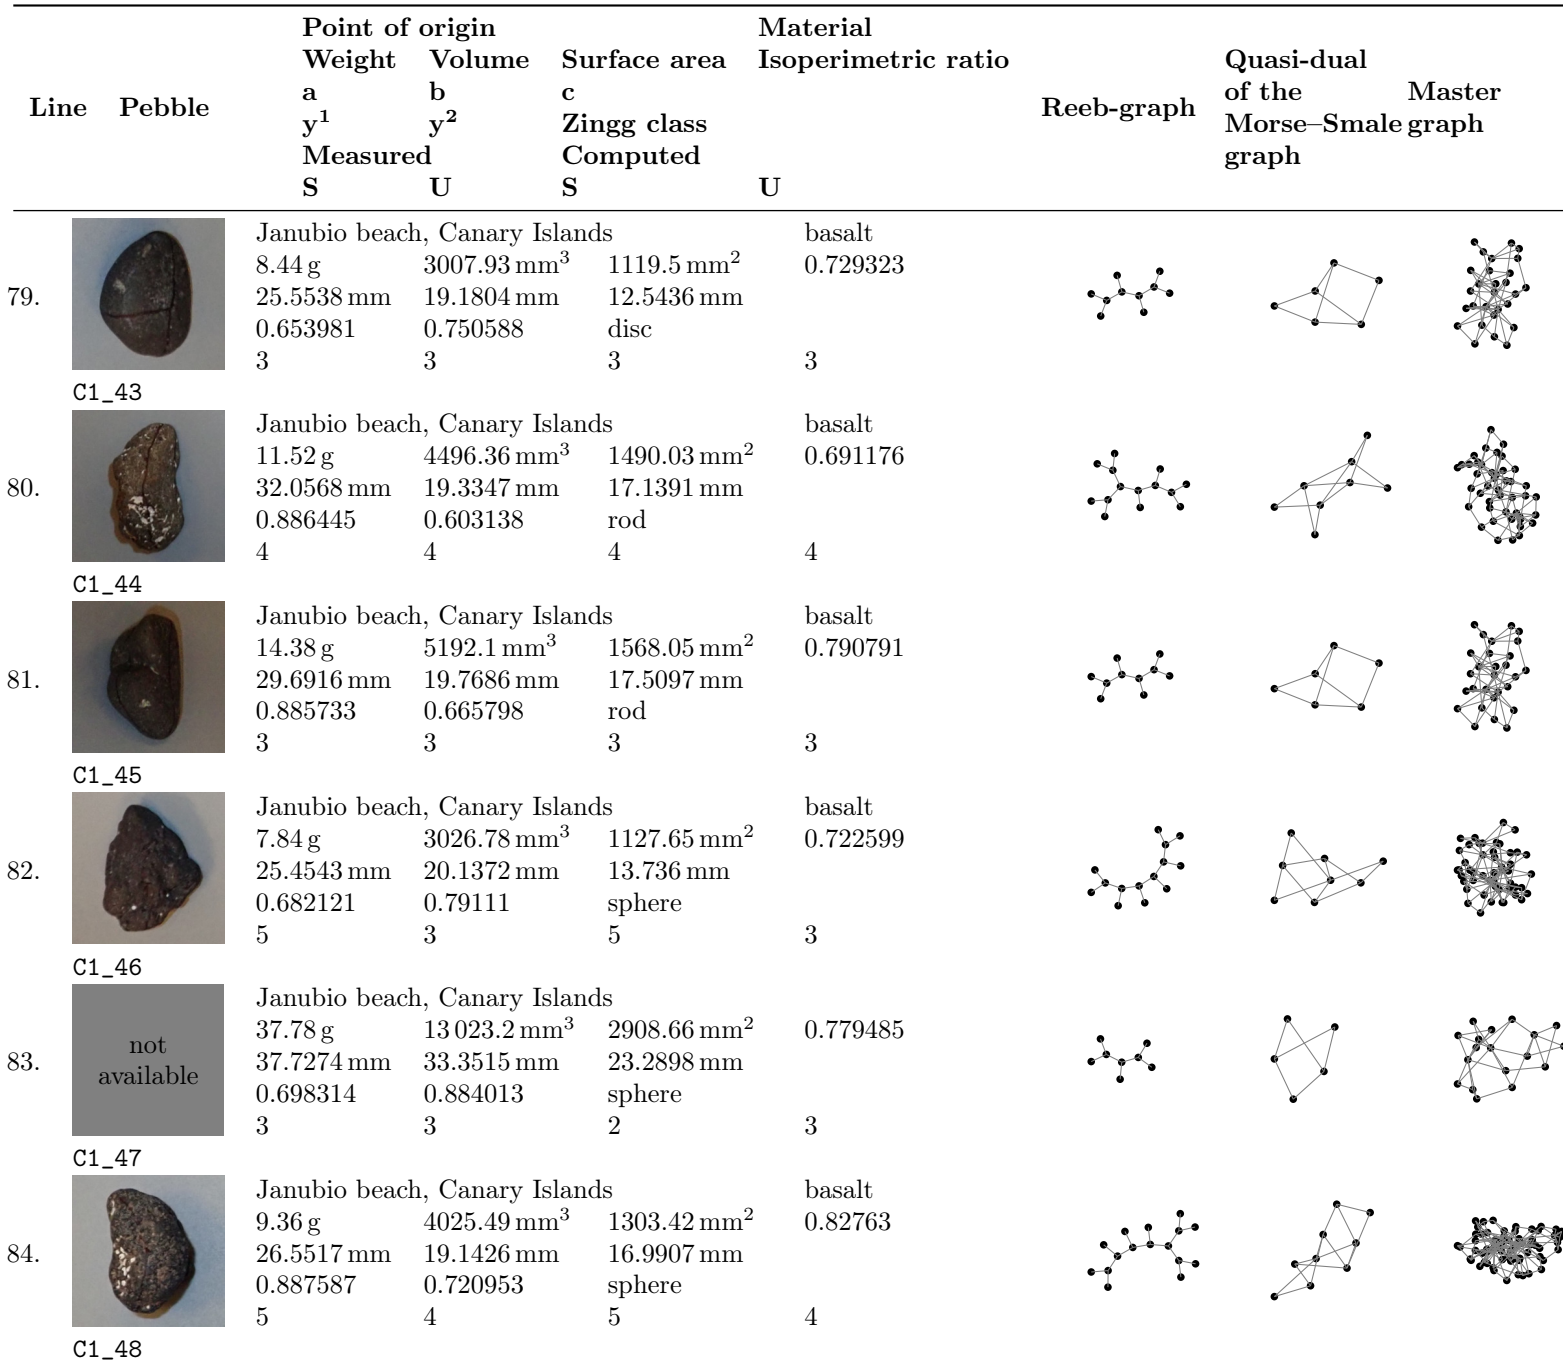   | 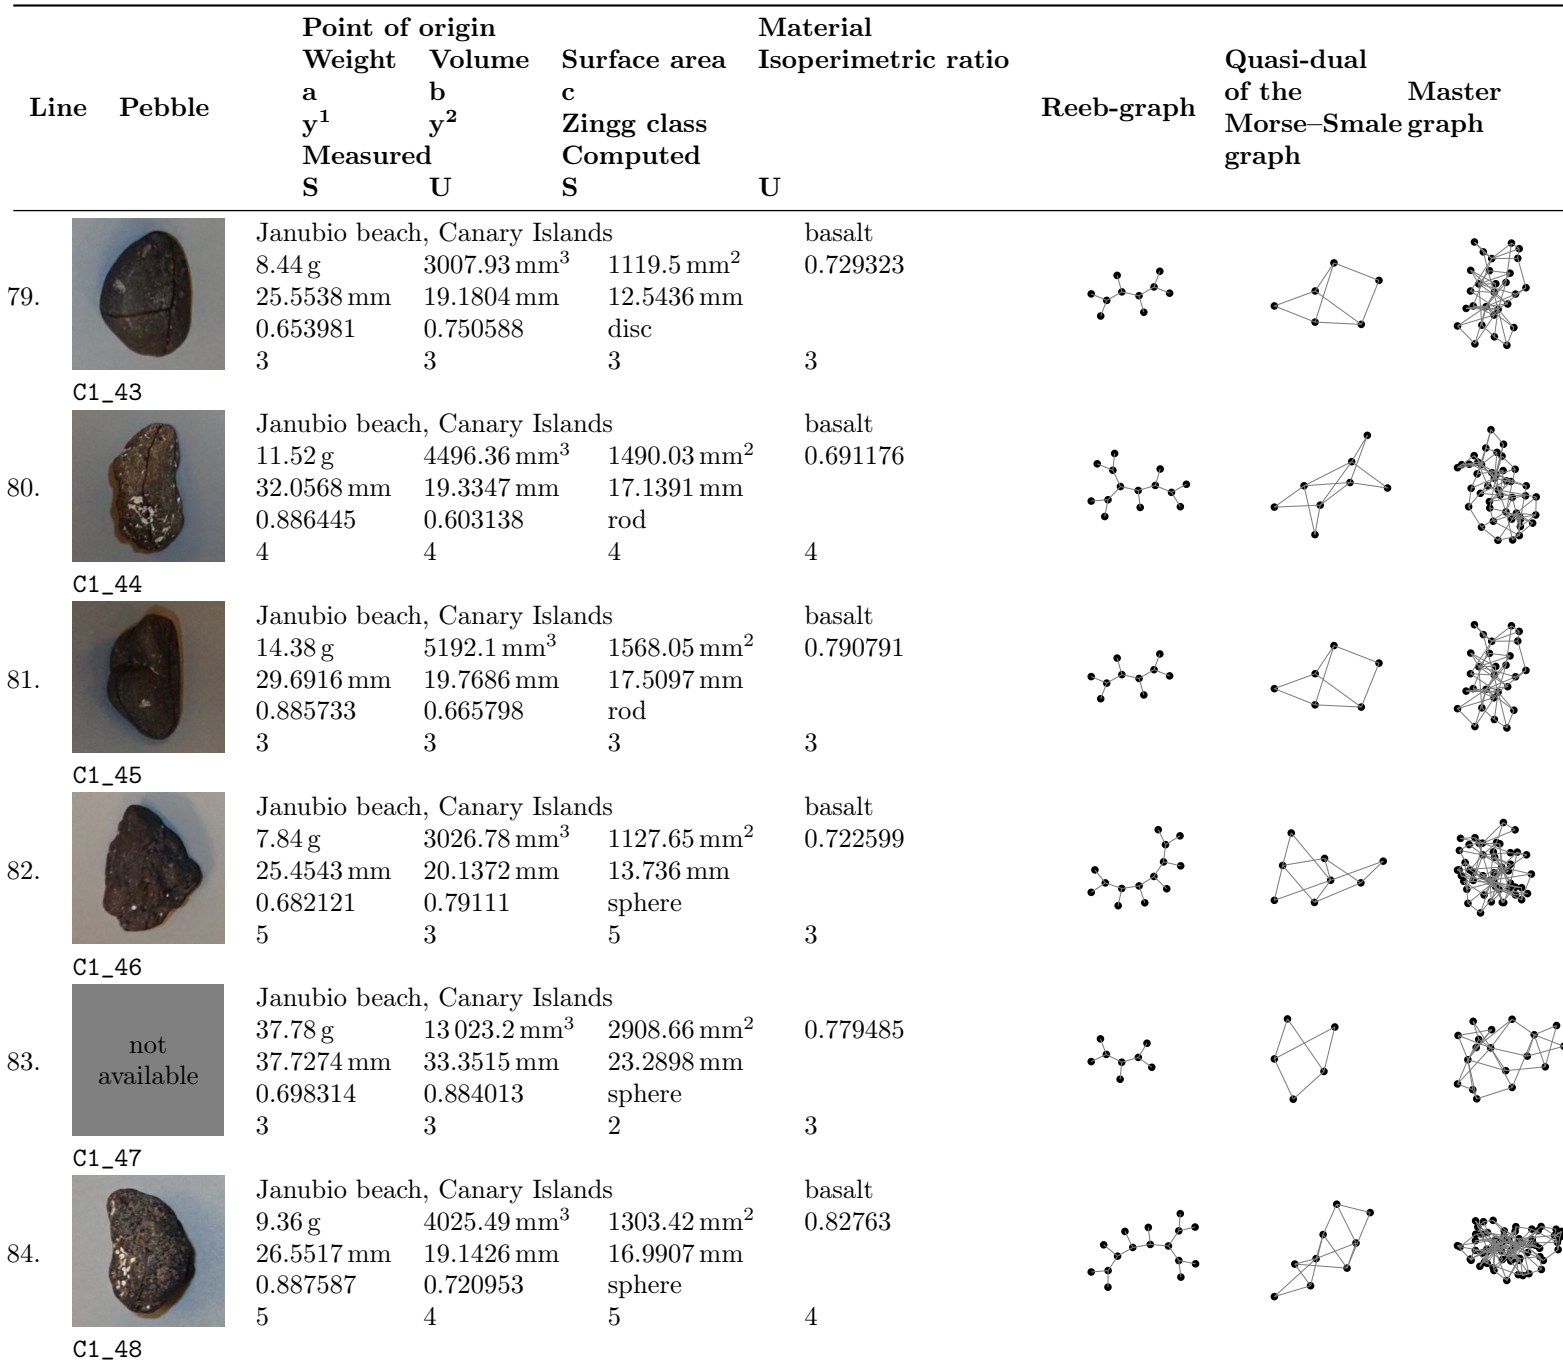   | 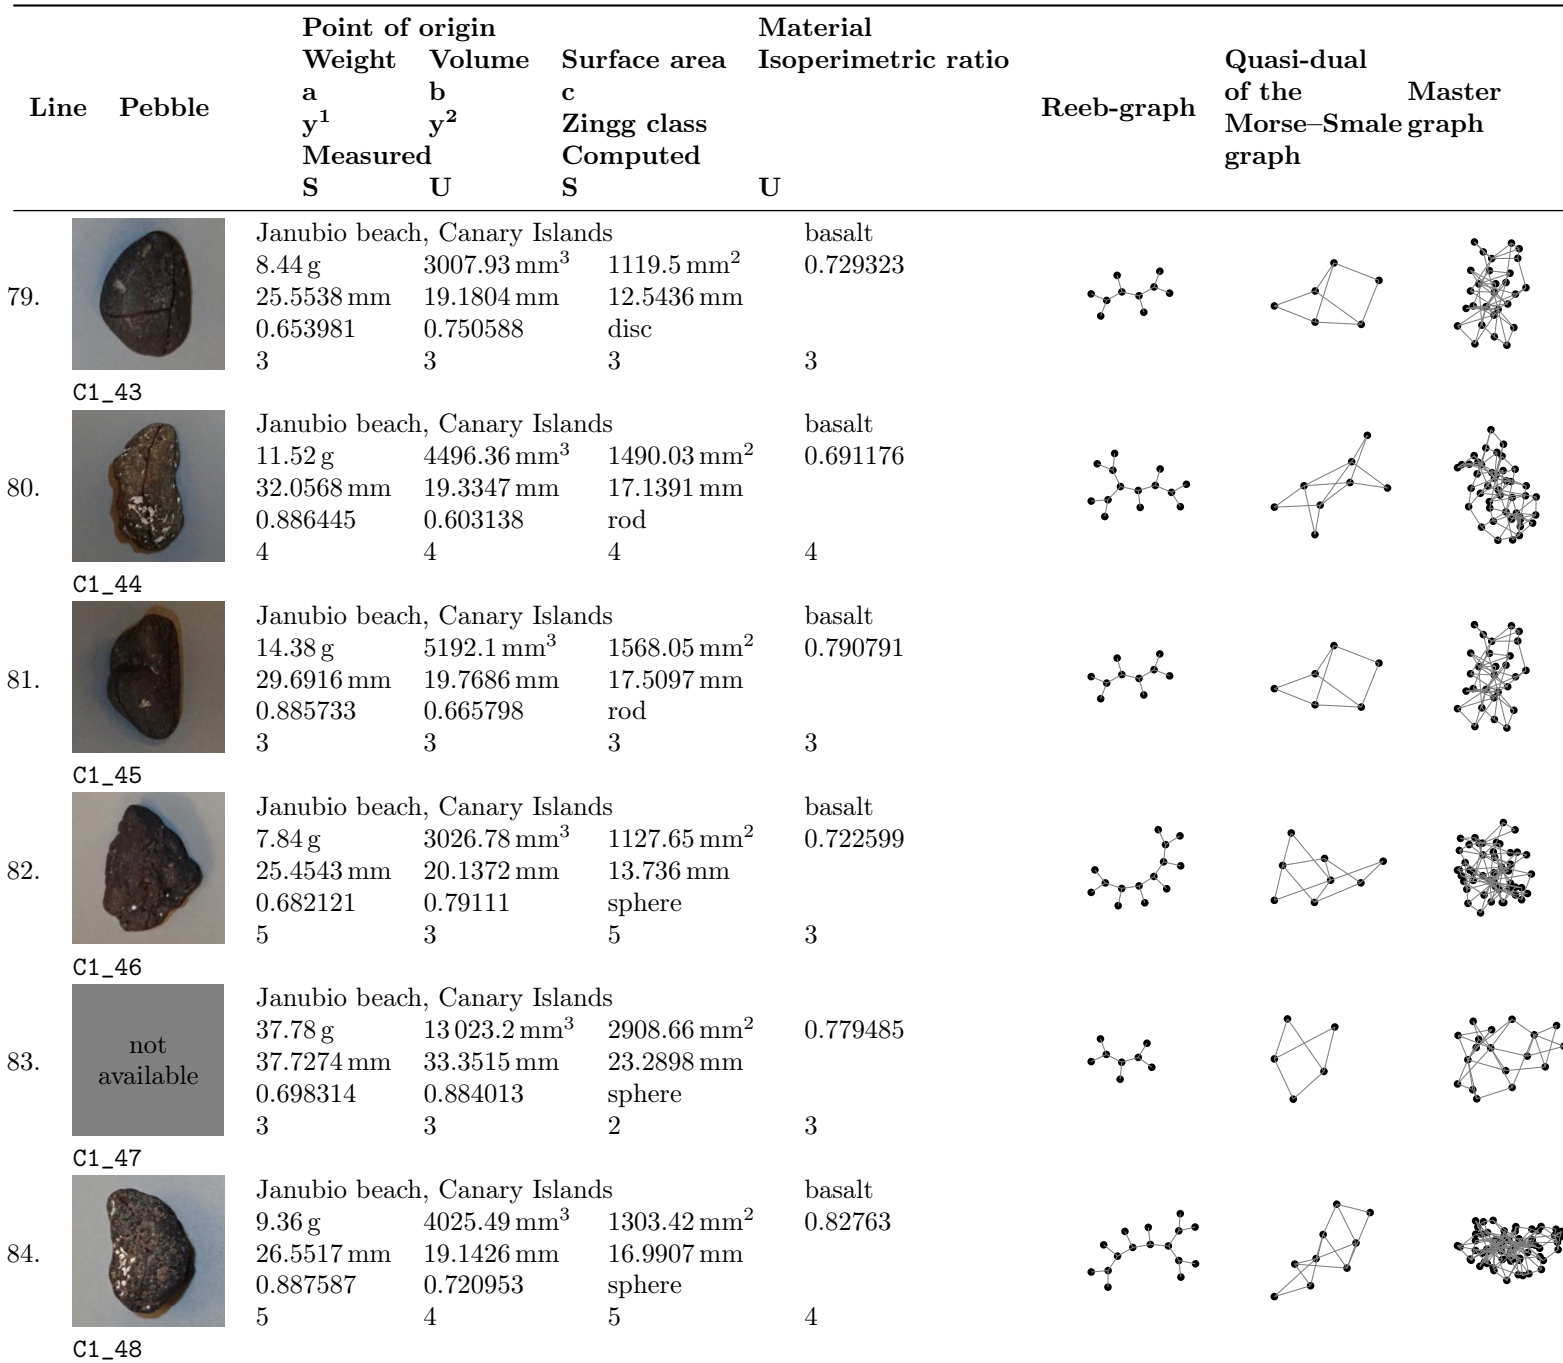   |
|      |                                                                                     | 11.52 g                         | 4496.36 mm <sup>3</sup>  | 1490.03 mm <sup>2</sup>      |          |                     |                                                                                       |                                                                                       |                                                                                       |
|      |                                                                                     | 32.0568 mm                      | 19.3347 mm               | 17.1391 mm                   |          |                     |                                                                                       |                                                                                       |                                                                                       |
|      |                                                                                     | 0.886445                        | 0.603138                 | rod                          |          |                     |                                                                                       |                                                                                       |                                                                                       |
|      |                                                                                     | 4                               | 4                        | 4                            |          |                     |                                                                                       |                                                                                       |                                                                                       |
|      | C1_44                                                                               |                                 |                          |                              |          |                     |                                                                                       |                                                                                       |                                                                                       |
| 81.  | 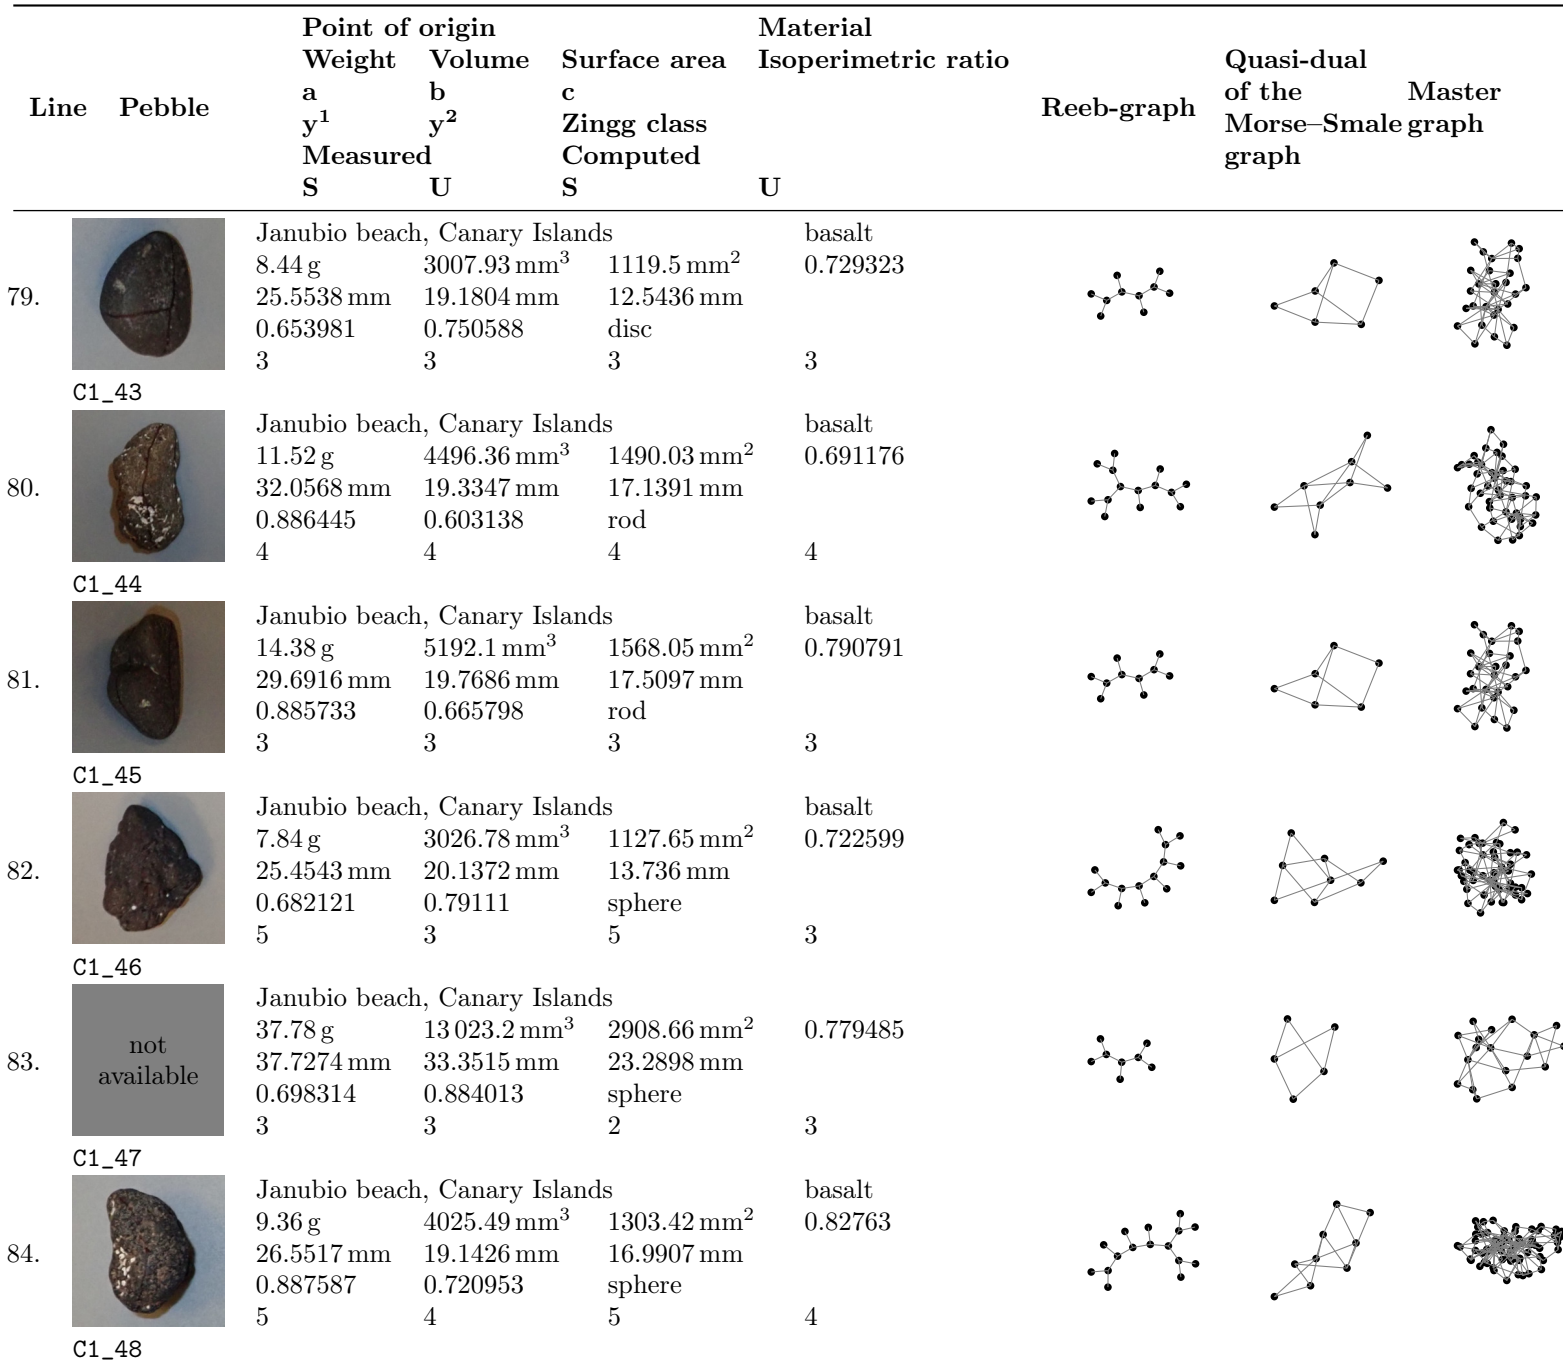   | Janubio beach, Canary Islands   |                          |                              | basalt   | 0.790791            | 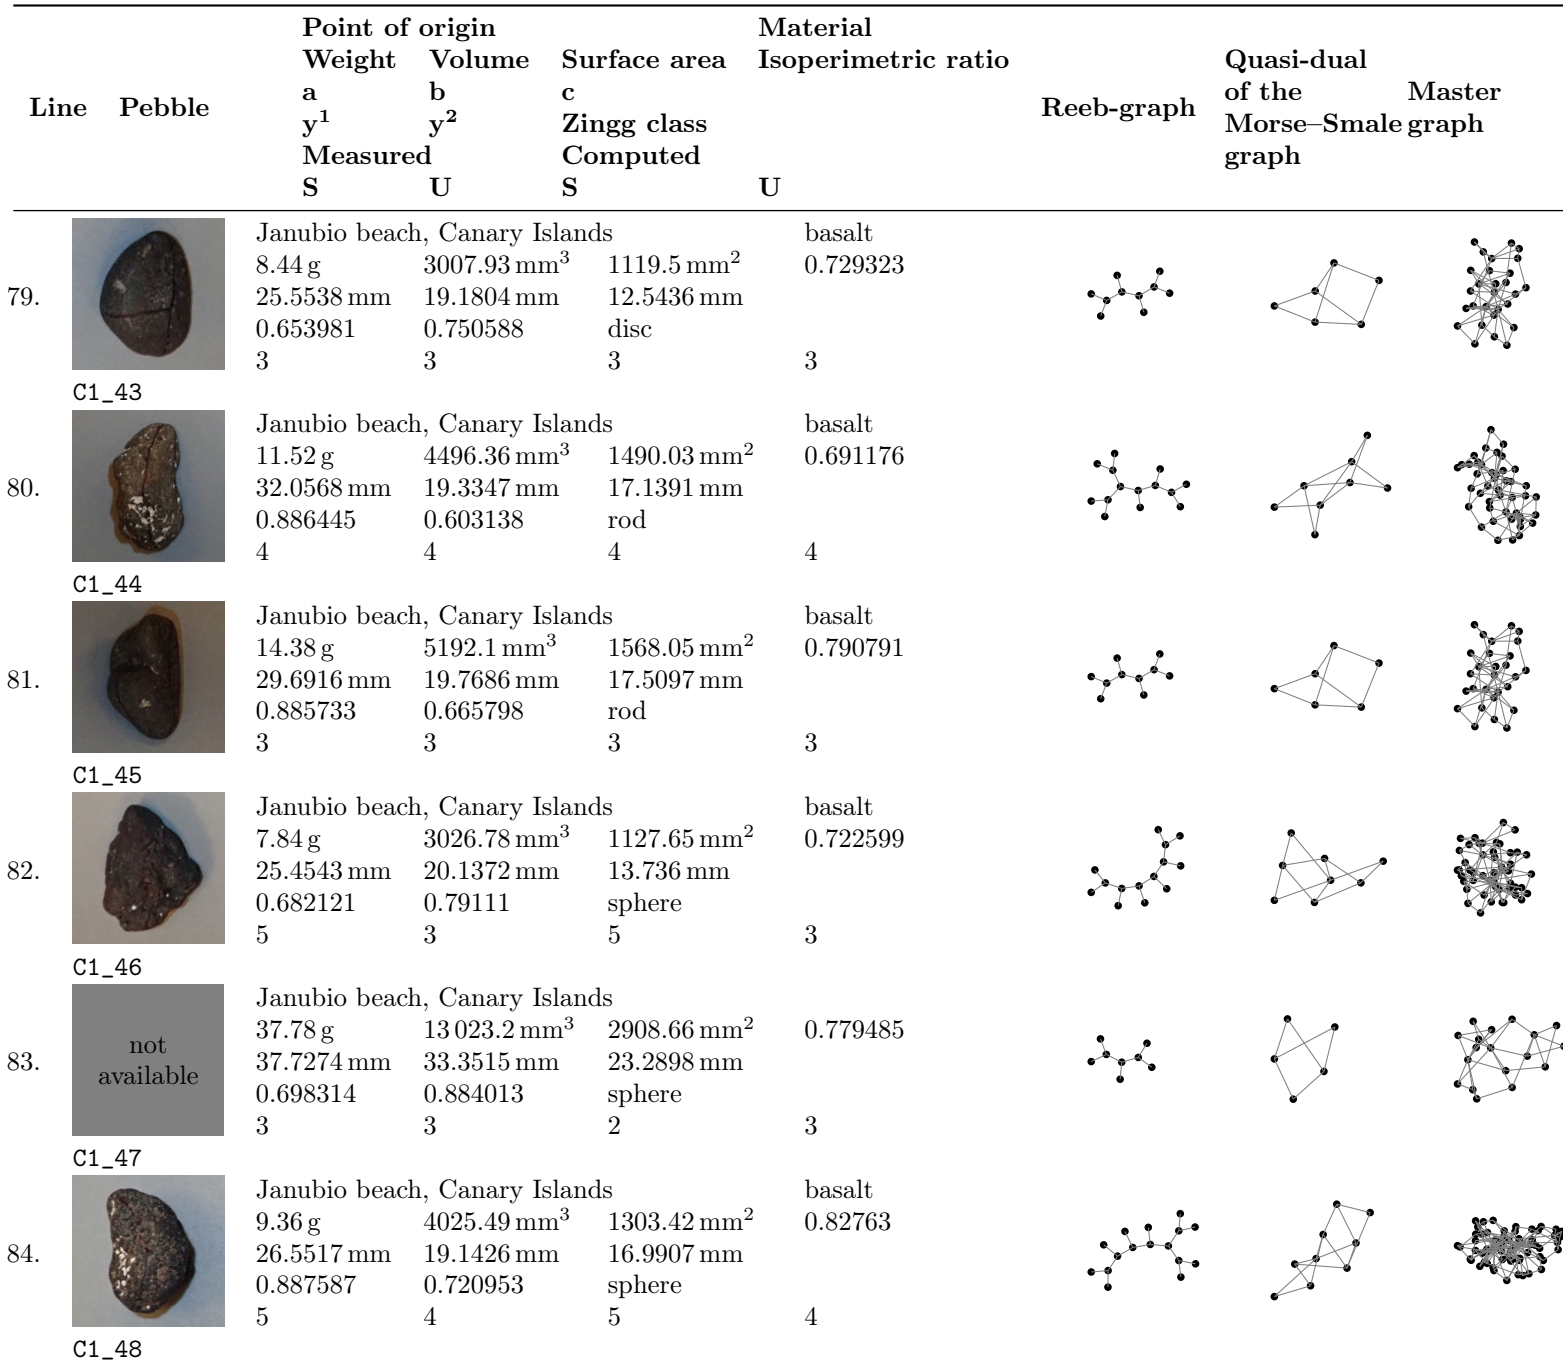   | 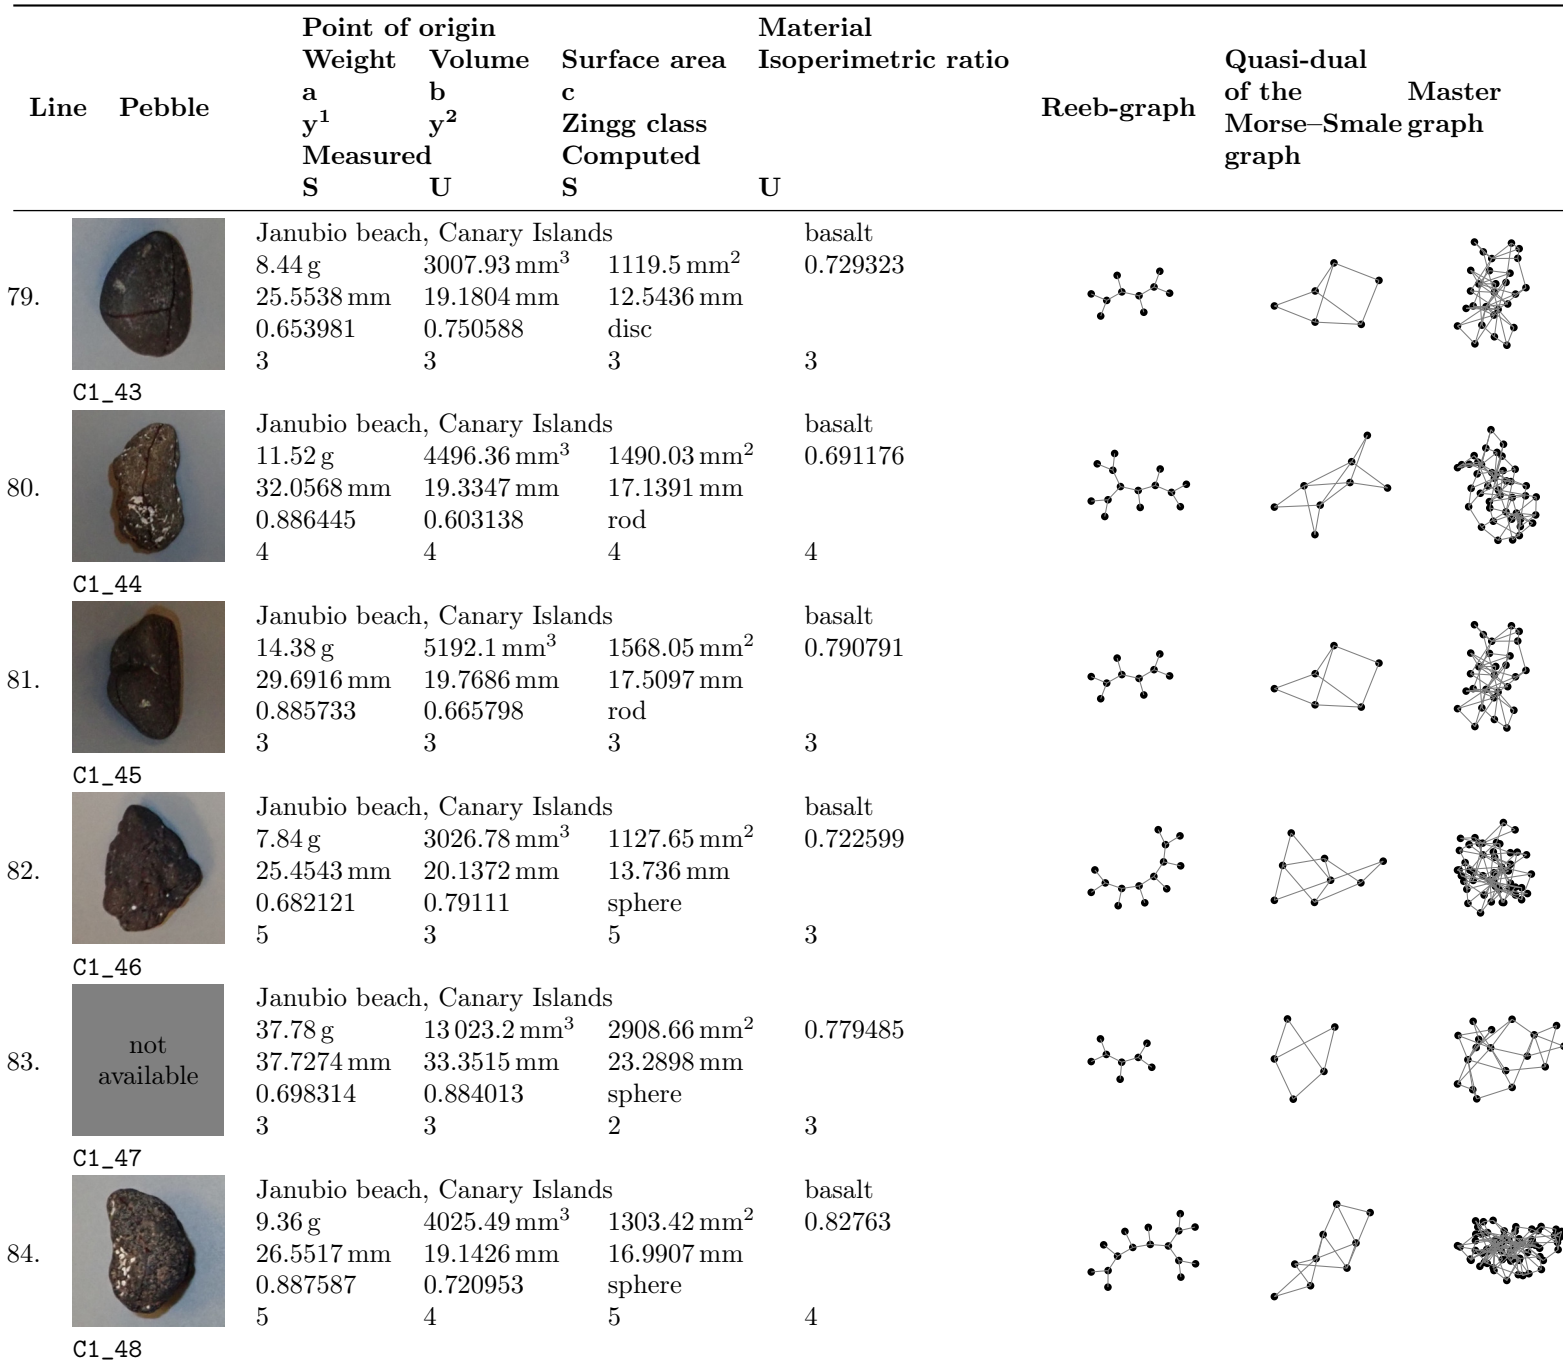   | 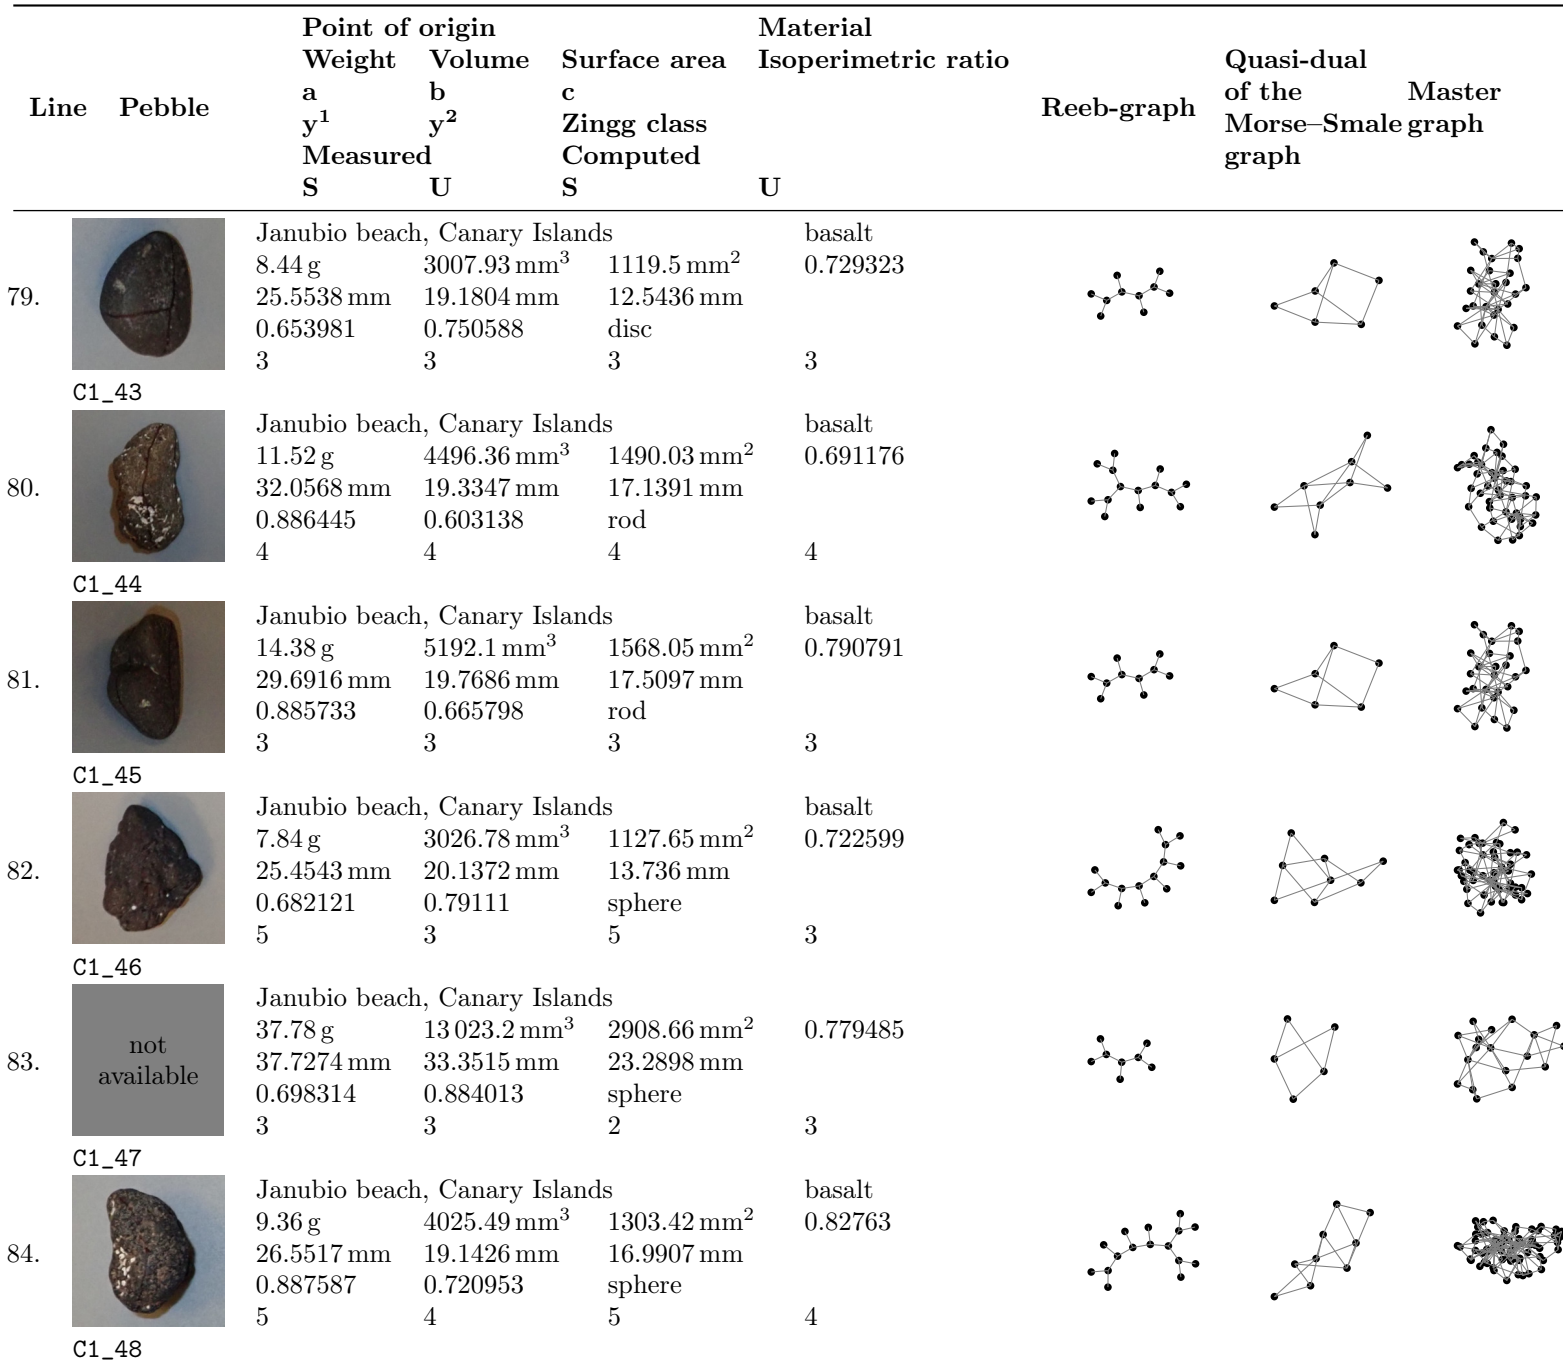   |
|      |                                                                                     | 14.38 g                         | 5192.1 mm <sup>3</sup>   | 1568.05 mm <sup>2</sup>      |          |                     |                                                                                       |                                                                                       |                                                                                       |
|      |                                                                                     | 29.6916 mm                      | 19.7686 mm               | 17.5097 mm                   |          |                     |                                                                                       |                                                                                       |                                                                                       |
|      |                                                                                     | 0.885733                        | 0.665798                 | rod                          |          |                     |                                                                                       |                                                                                       |                                                                                       |
|      |                                                                                     | 3                               | 3                        | 3                            |          |                     |                                                                                       |                                                                                       |                                                                                       |
|      | C1_45                                                                               |                                 |                          |                              |          |                     |                                                                                       |                                                                                       |                                                                                       |
| 82.  | 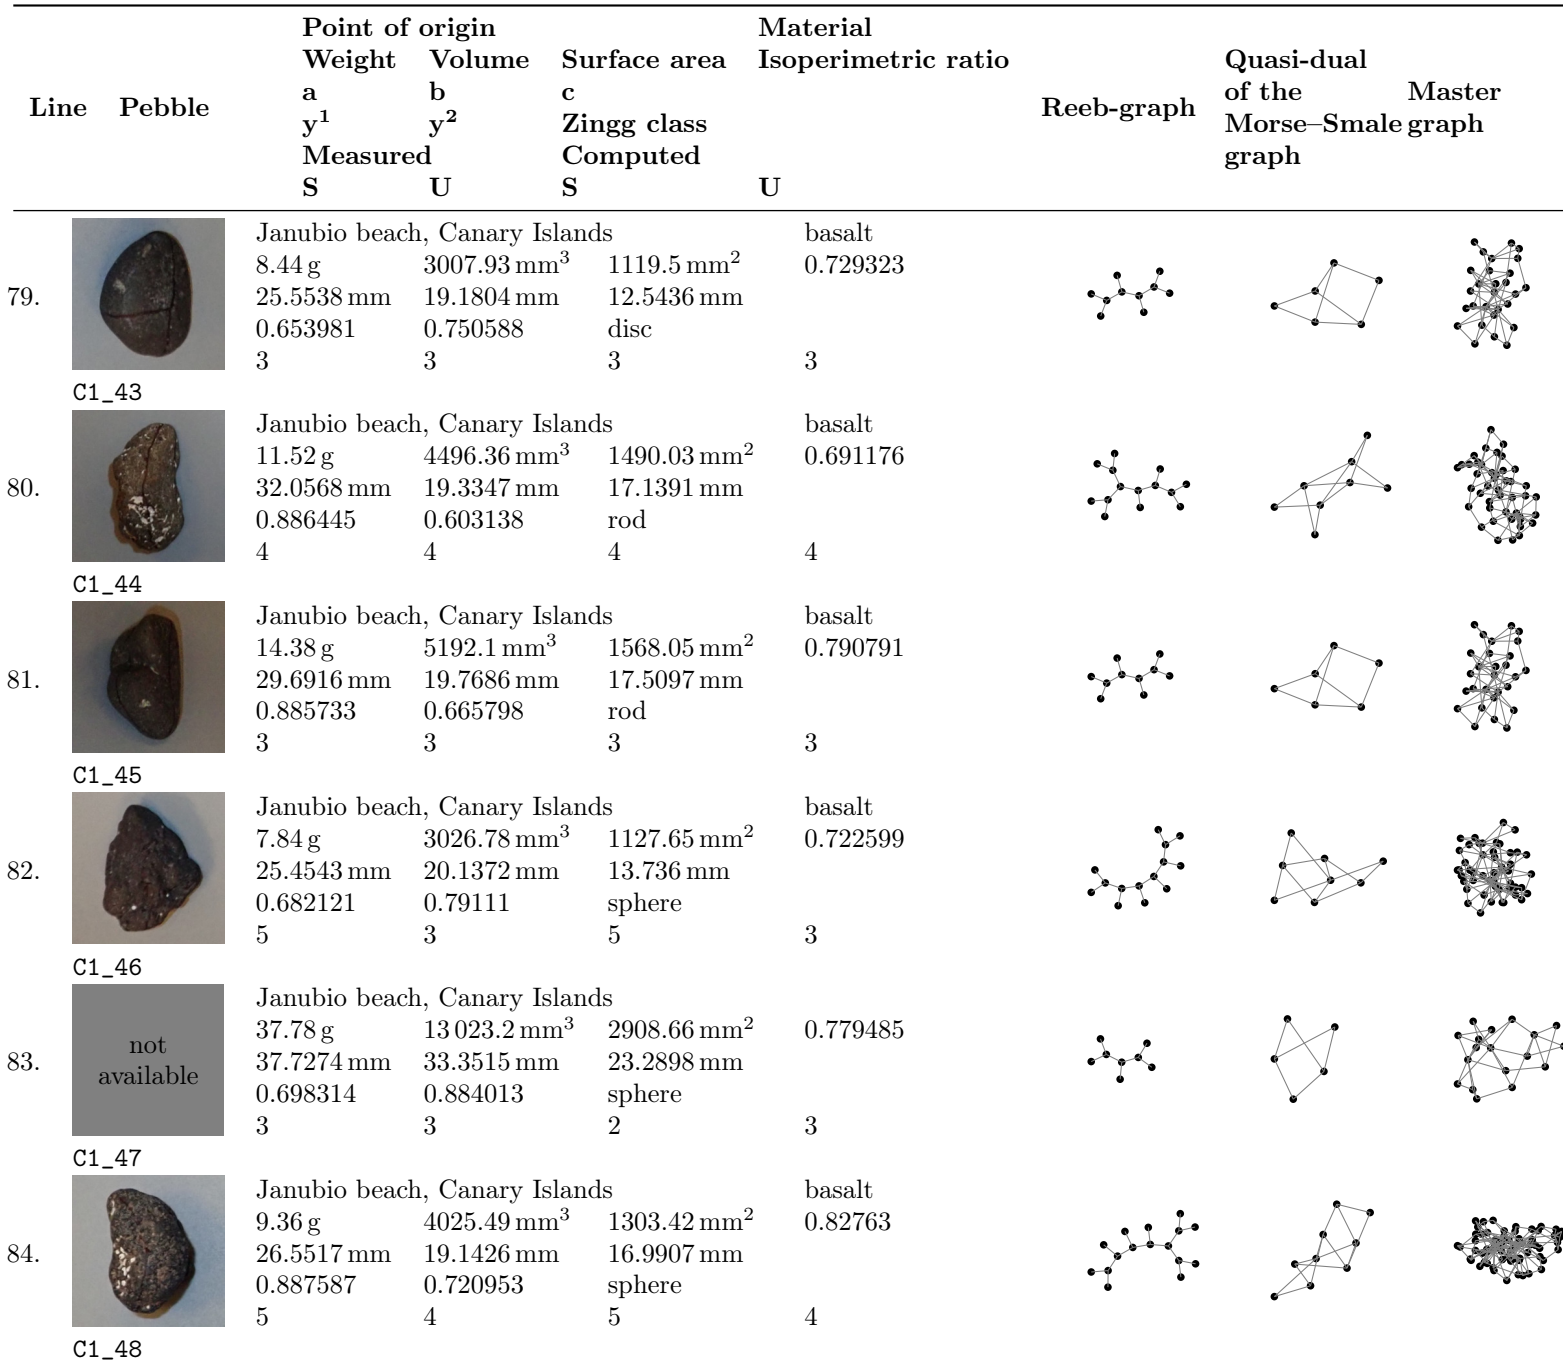  | Janubio beach, Canary Islands   |                          |                              | basalt   | 0.722599            | 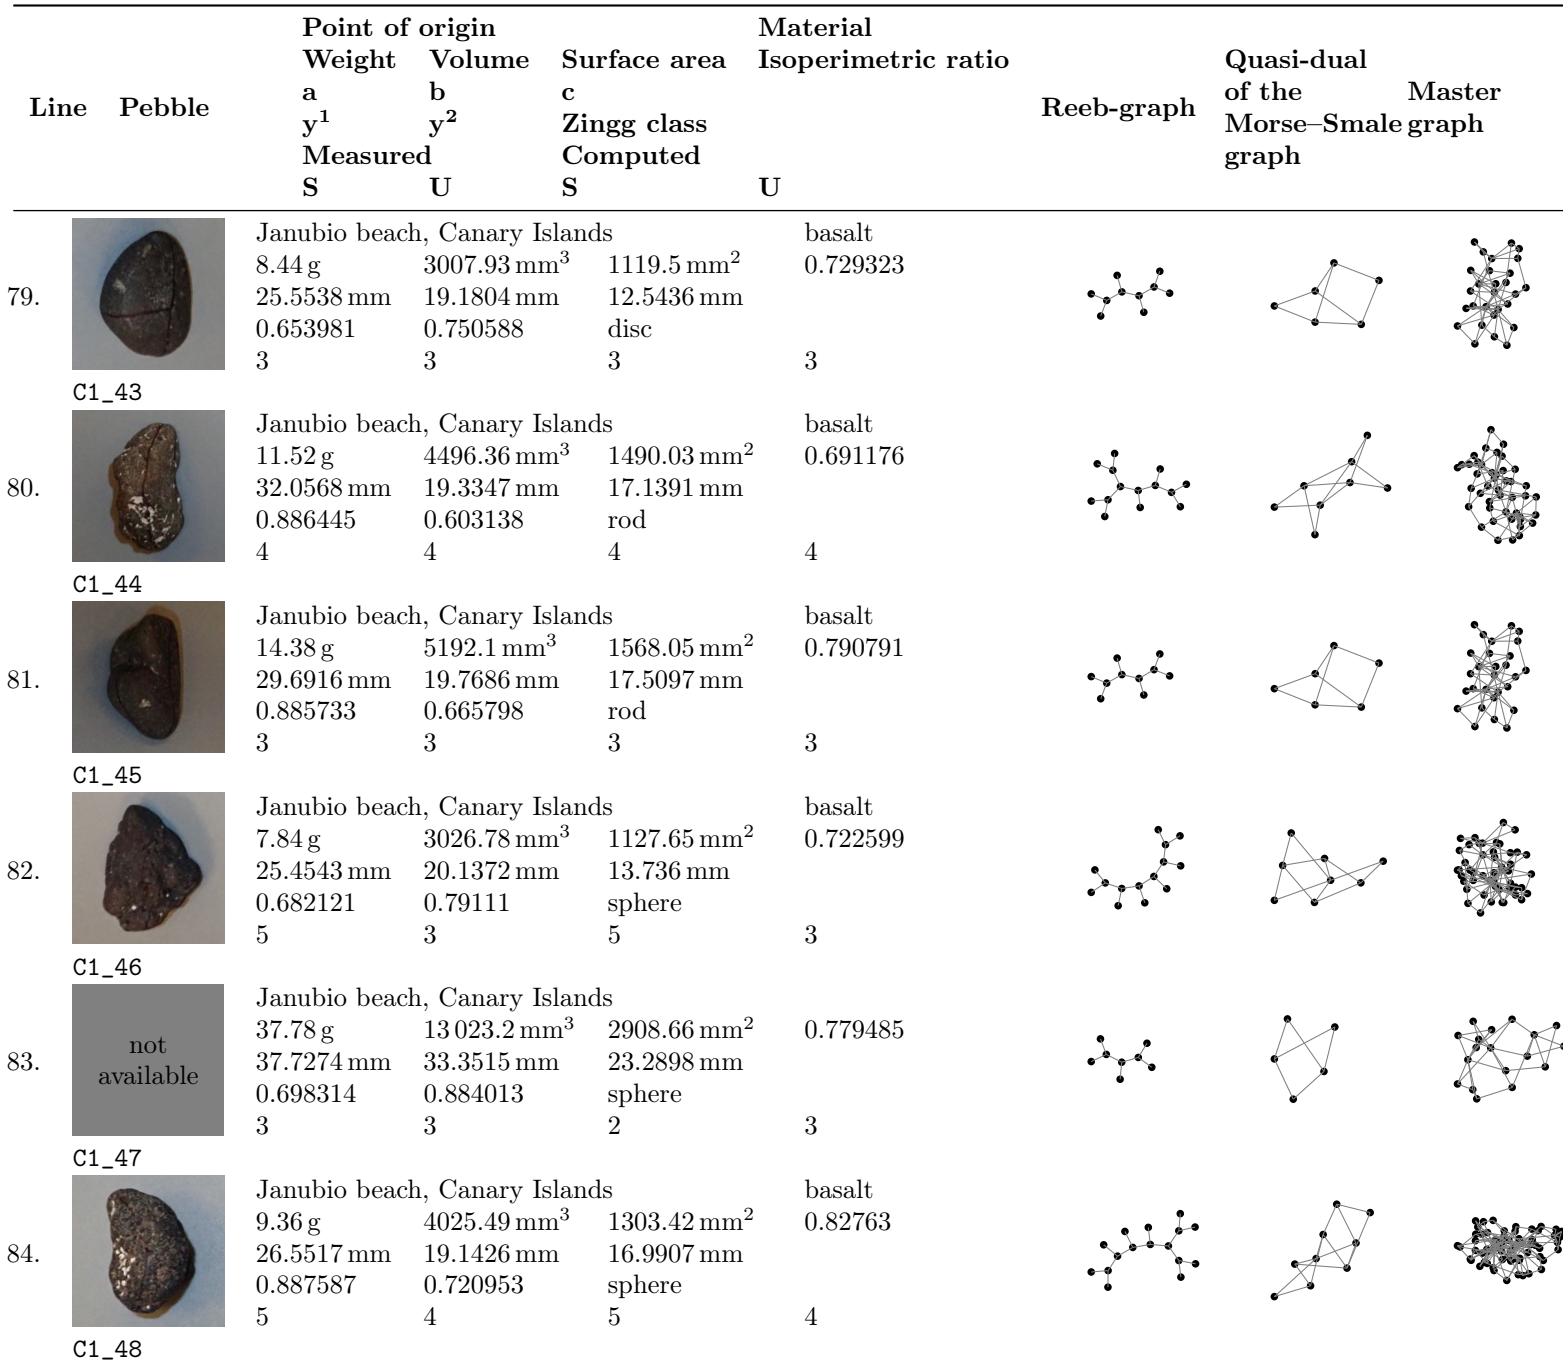  | 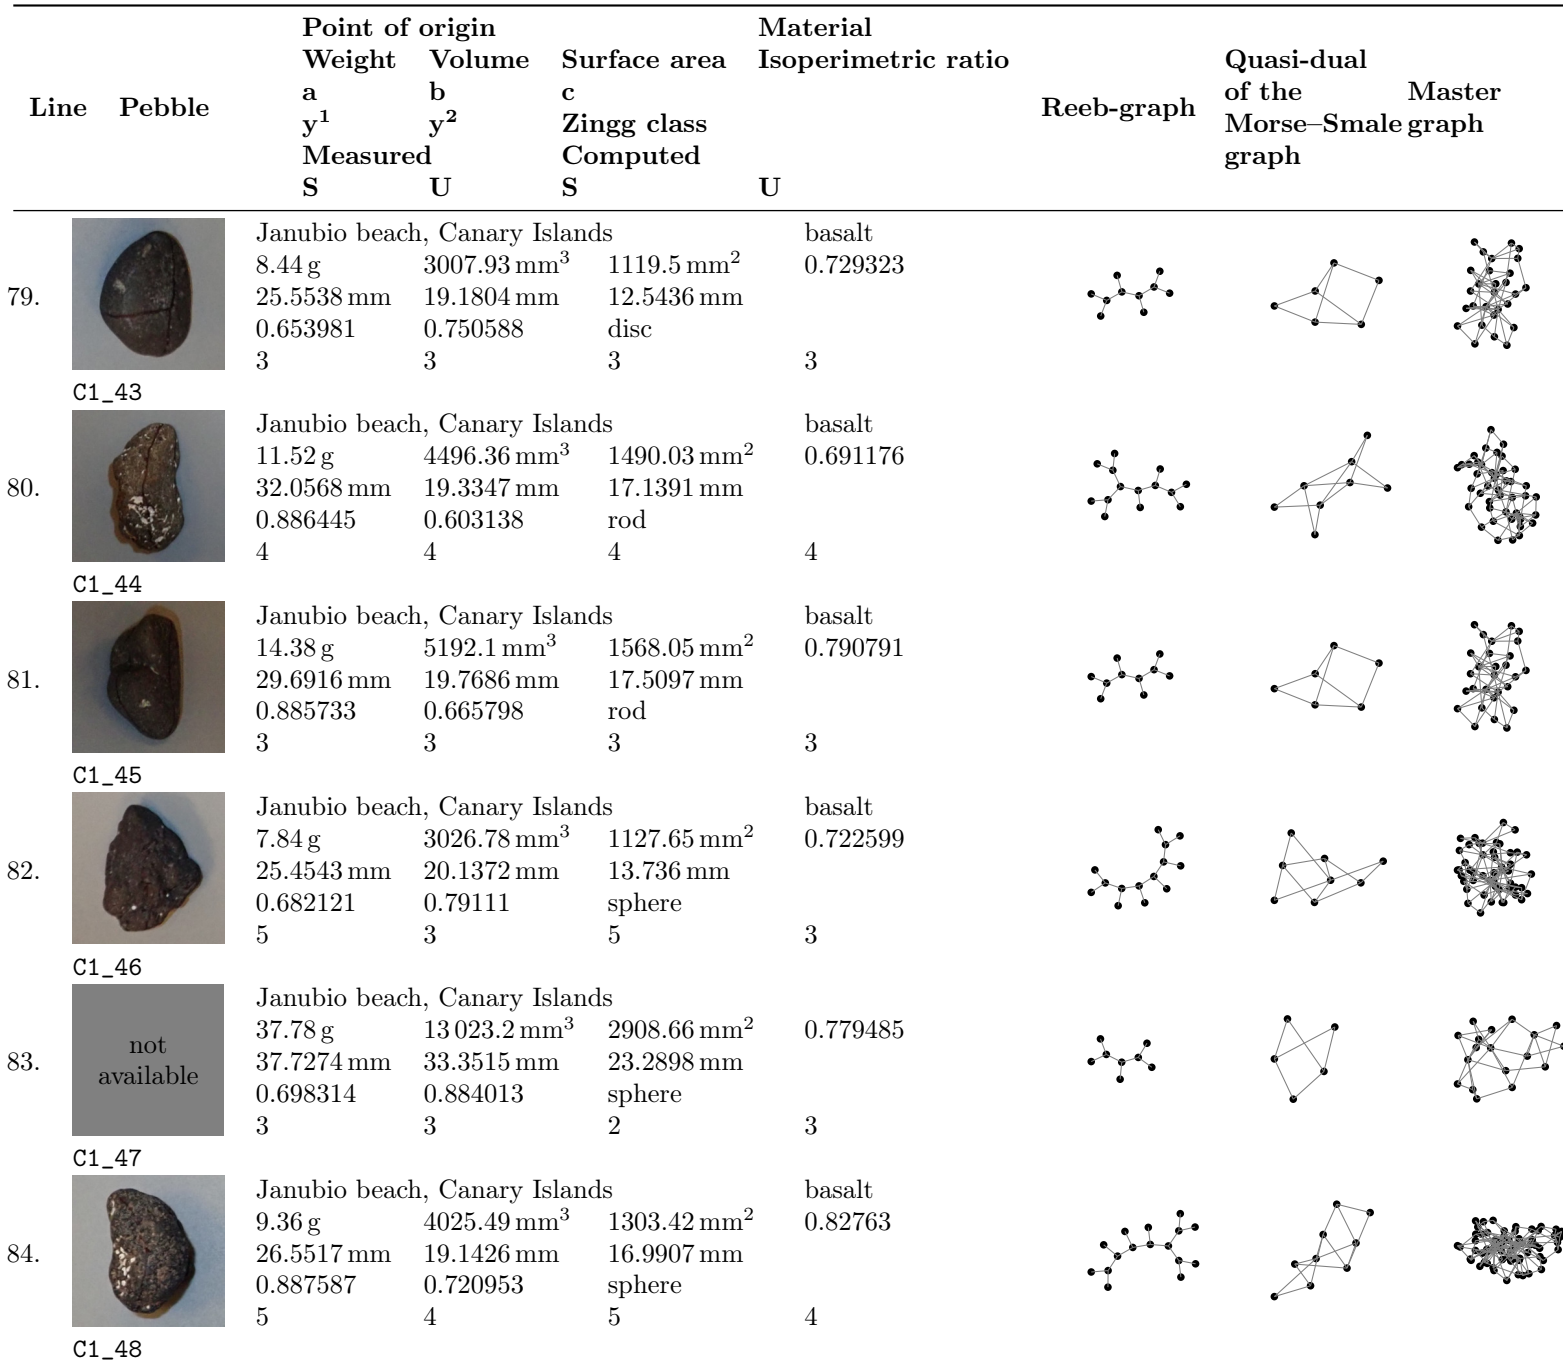  | 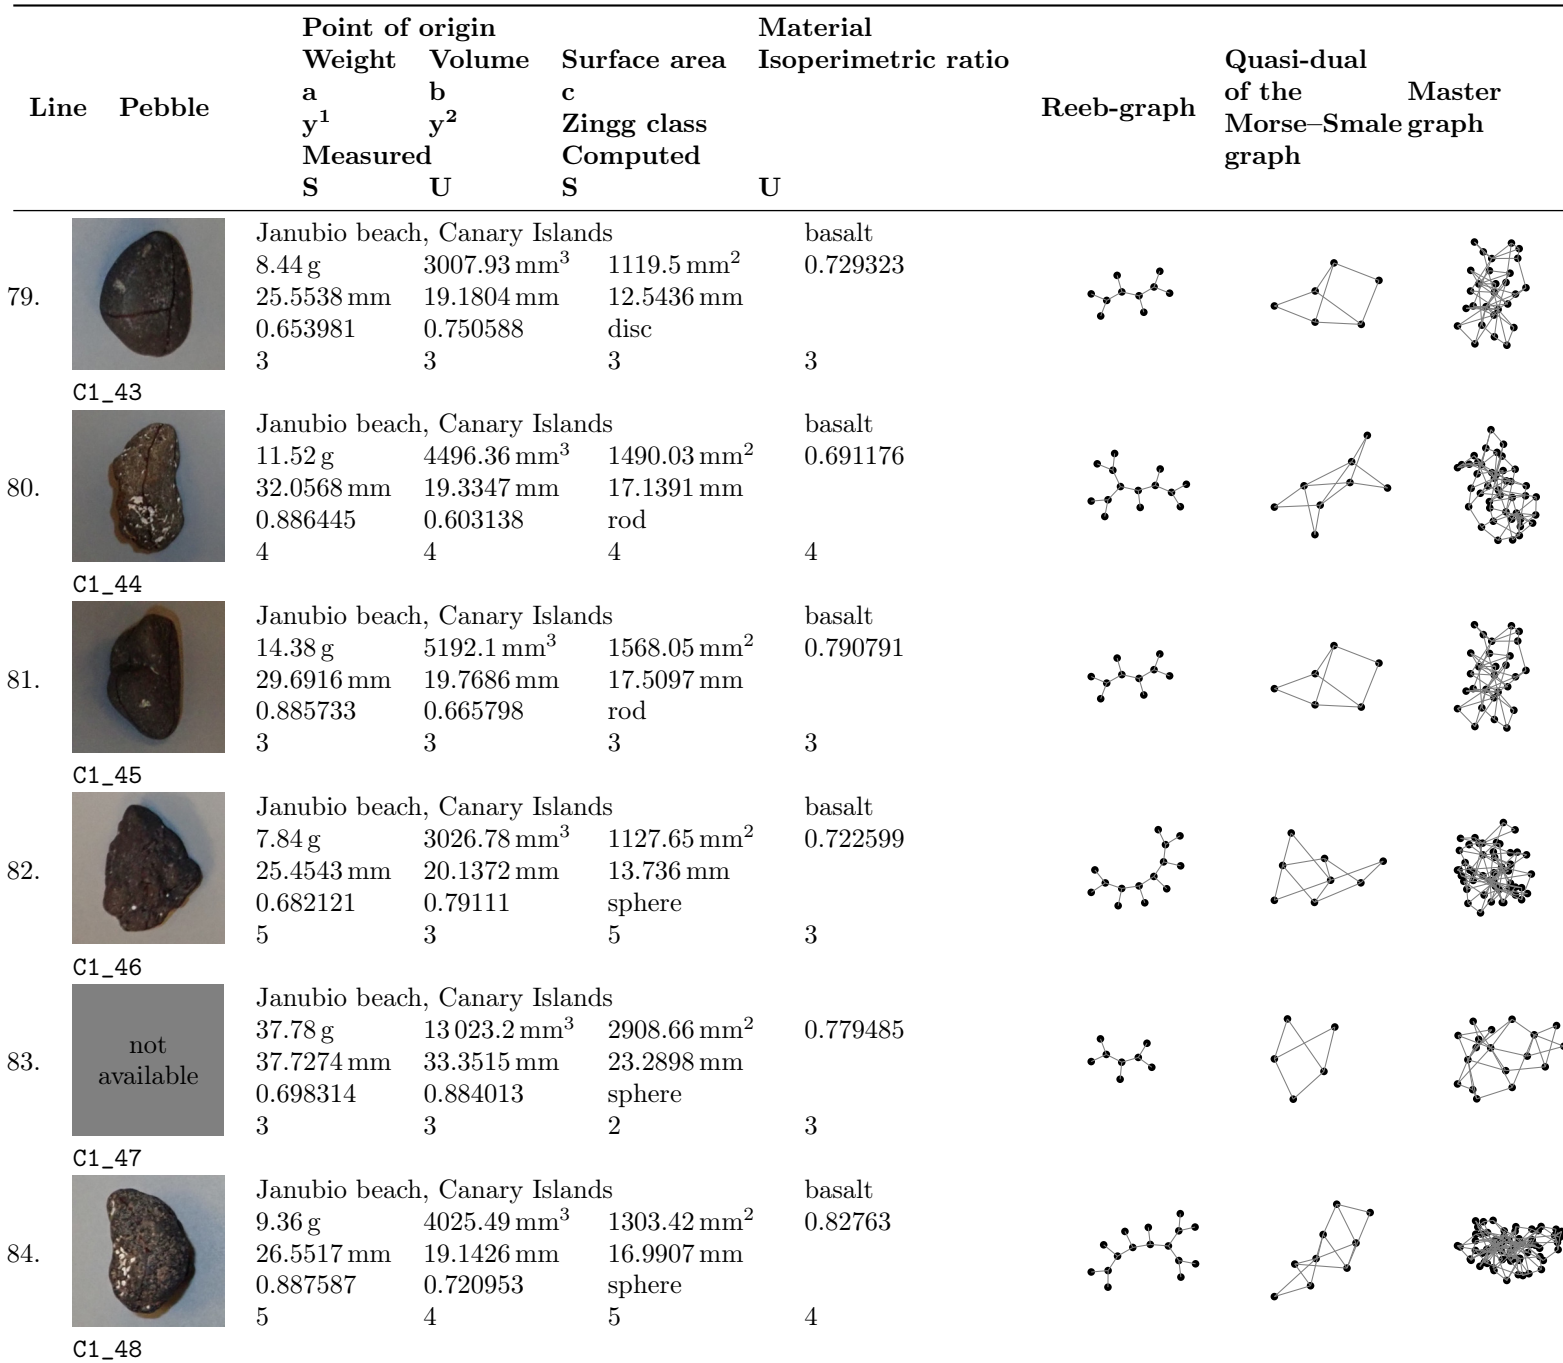  |
|      |                                                                                     | 7.84 g                          | 3026.78 mm <sup>3</sup>  | 1127.65 mm <sup>2</sup>      |          |                     |                                                                                       |                                                                                       |                                                                                       |
|      |                                                                                     | 25.4543 mm                      | 20.1372 mm               | 13.736 mm                    |          |                     |                                                                                       |                                                                                       |                                                                                       |
|      |                                                                                     | 0.682121                        | 0.79111                  | sphere                       |          |                     |                                                                                       |                                                                                       |                                                                                       |
|      |                                                                                     | 5                               | 3                        | 5                            |          |                     |                                                                                       |                                                                                       |                                                                                       |
|      | C1_46                                                                               |                                 |                          |                              |          |                     |                                                                                       |                                                                                       |                                                                                       |
| 83.  | 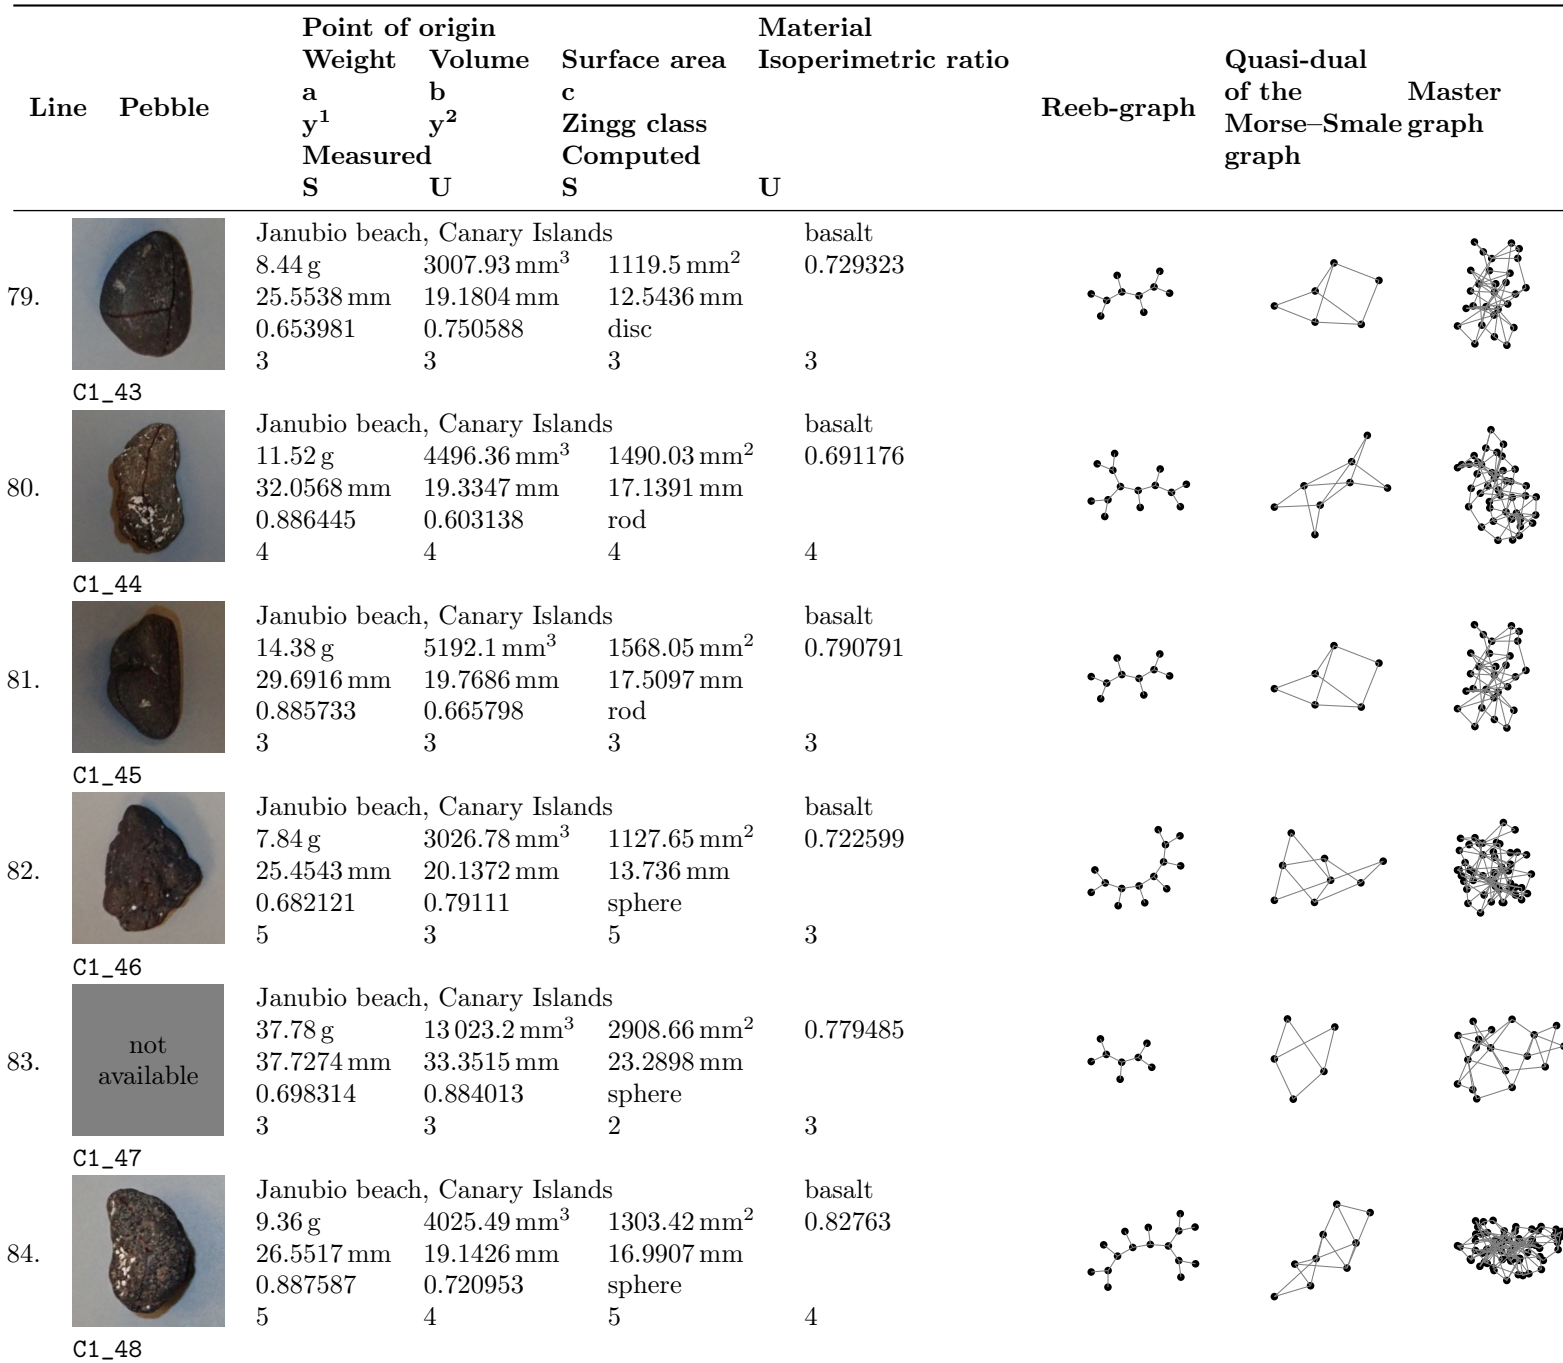 | Janubio beach, Canary Islands   |                          |                              | basalt   | 0.779485            | 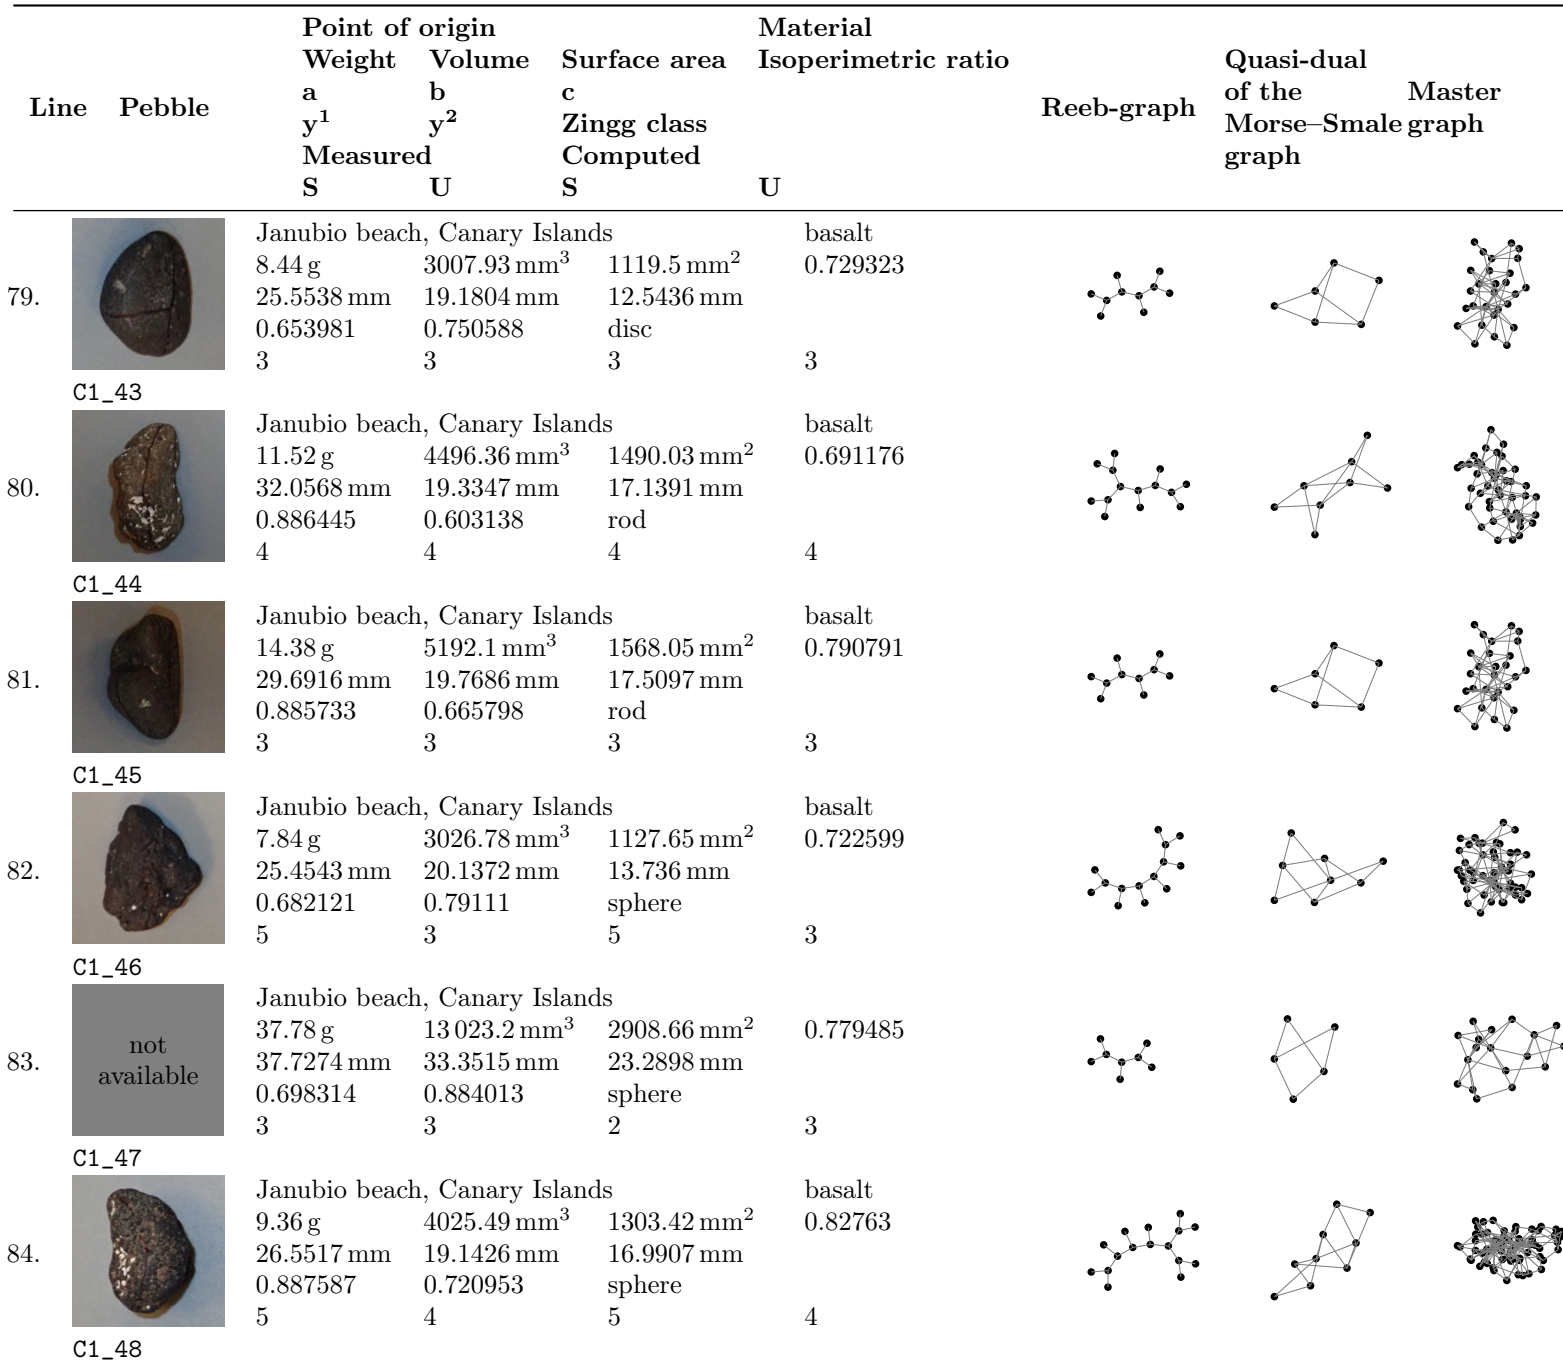 | 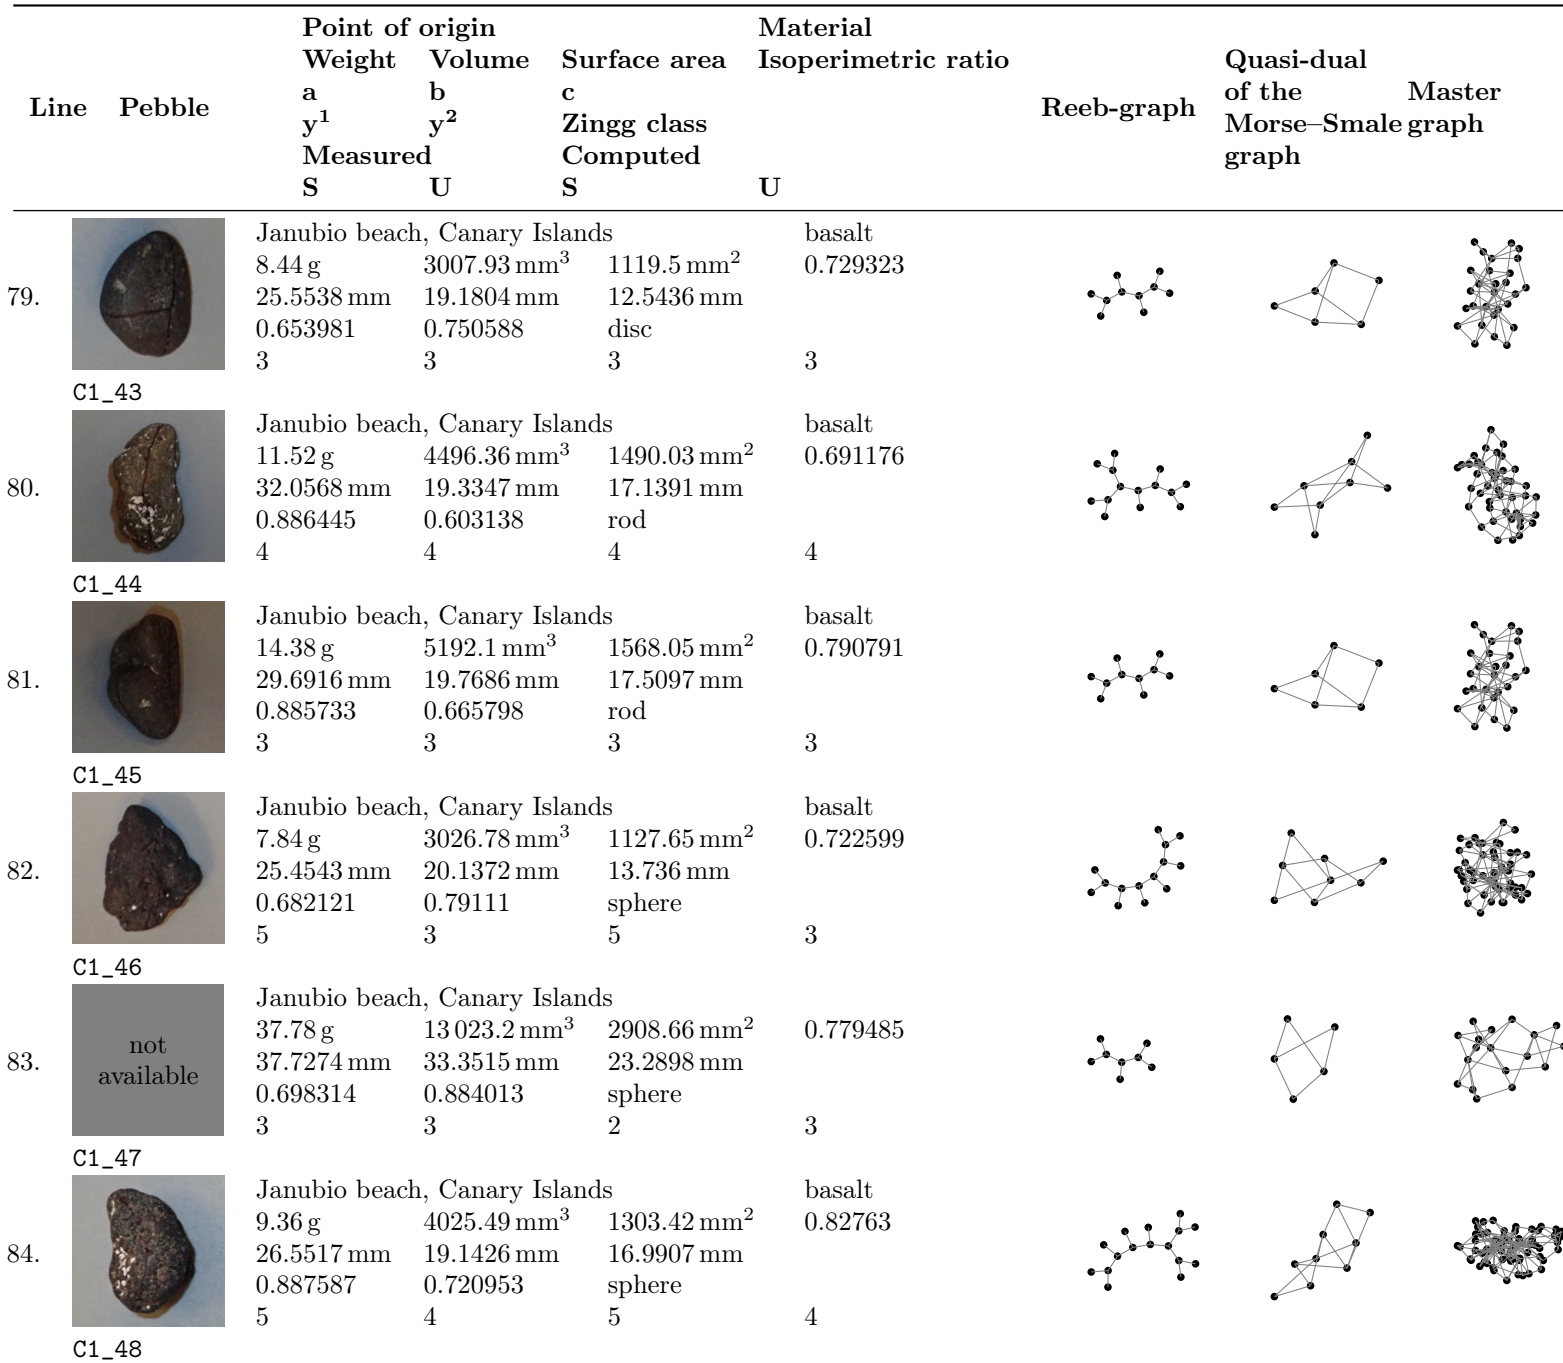 | 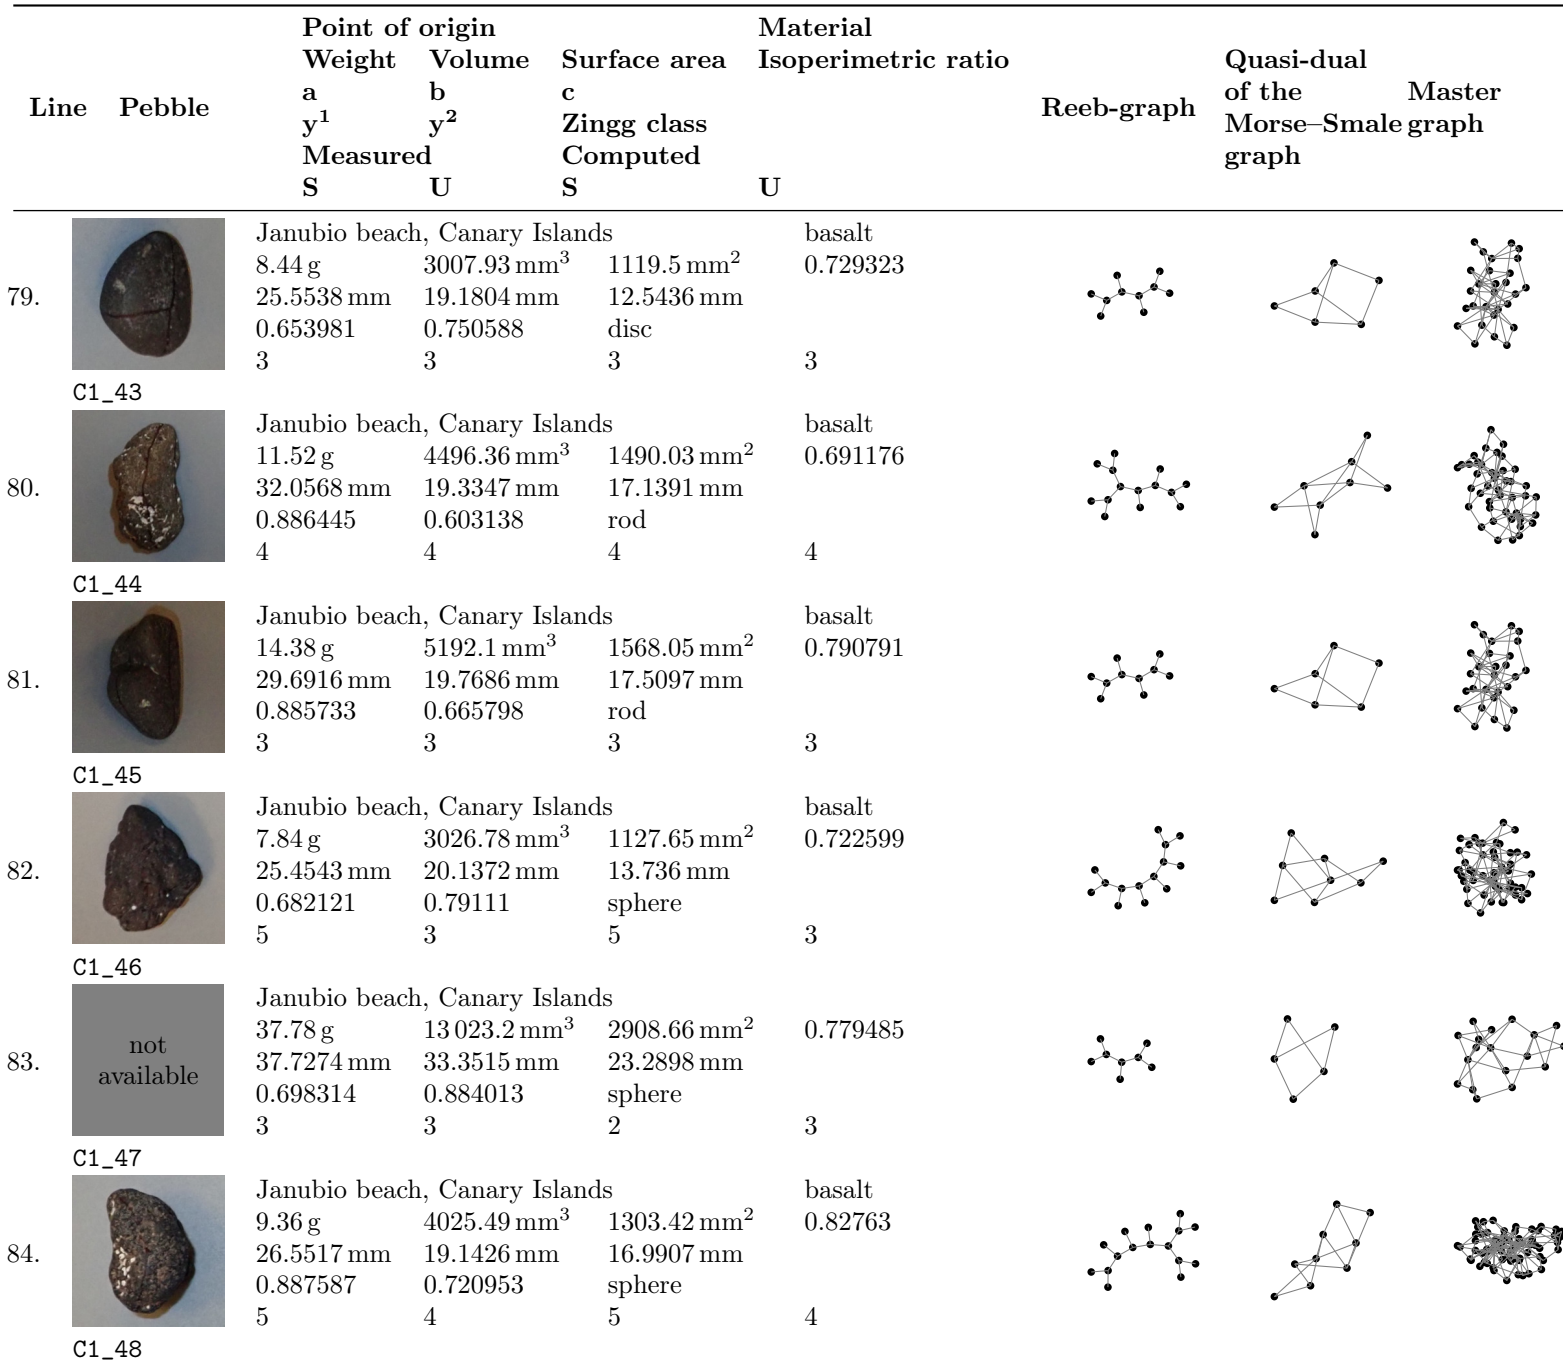 |
|      |                                                                                     | 37.78 g                         | 13 023.2 mm <sup>3</sup> | 2908.66 mm <sup>2</sup>      |          |                     |                                                                                       |                                                                                       |                                                                                       |
|      |                                                                                     | 37.7274 mm                      | 33.3515 mm               | 23.2898 mm                   |          |                     |                                                                                       |                                                                                       |                                                                                       |
|      |                                                                                     | 0.698314                        | 0.884013                 | sphere                       |          |                     |                                                                                       |                                                                                       |                                                                                       |
|      |                                                                                     | 3                               | 3                        | 2                            |          |                     |                                                                                       |                                                                                       |                                                                                       |
|      | C1_47                                                                               |                                 |                          |                              |          |                     |                                                                                       |                                                                                       |                                                                                       |
| 84.  | 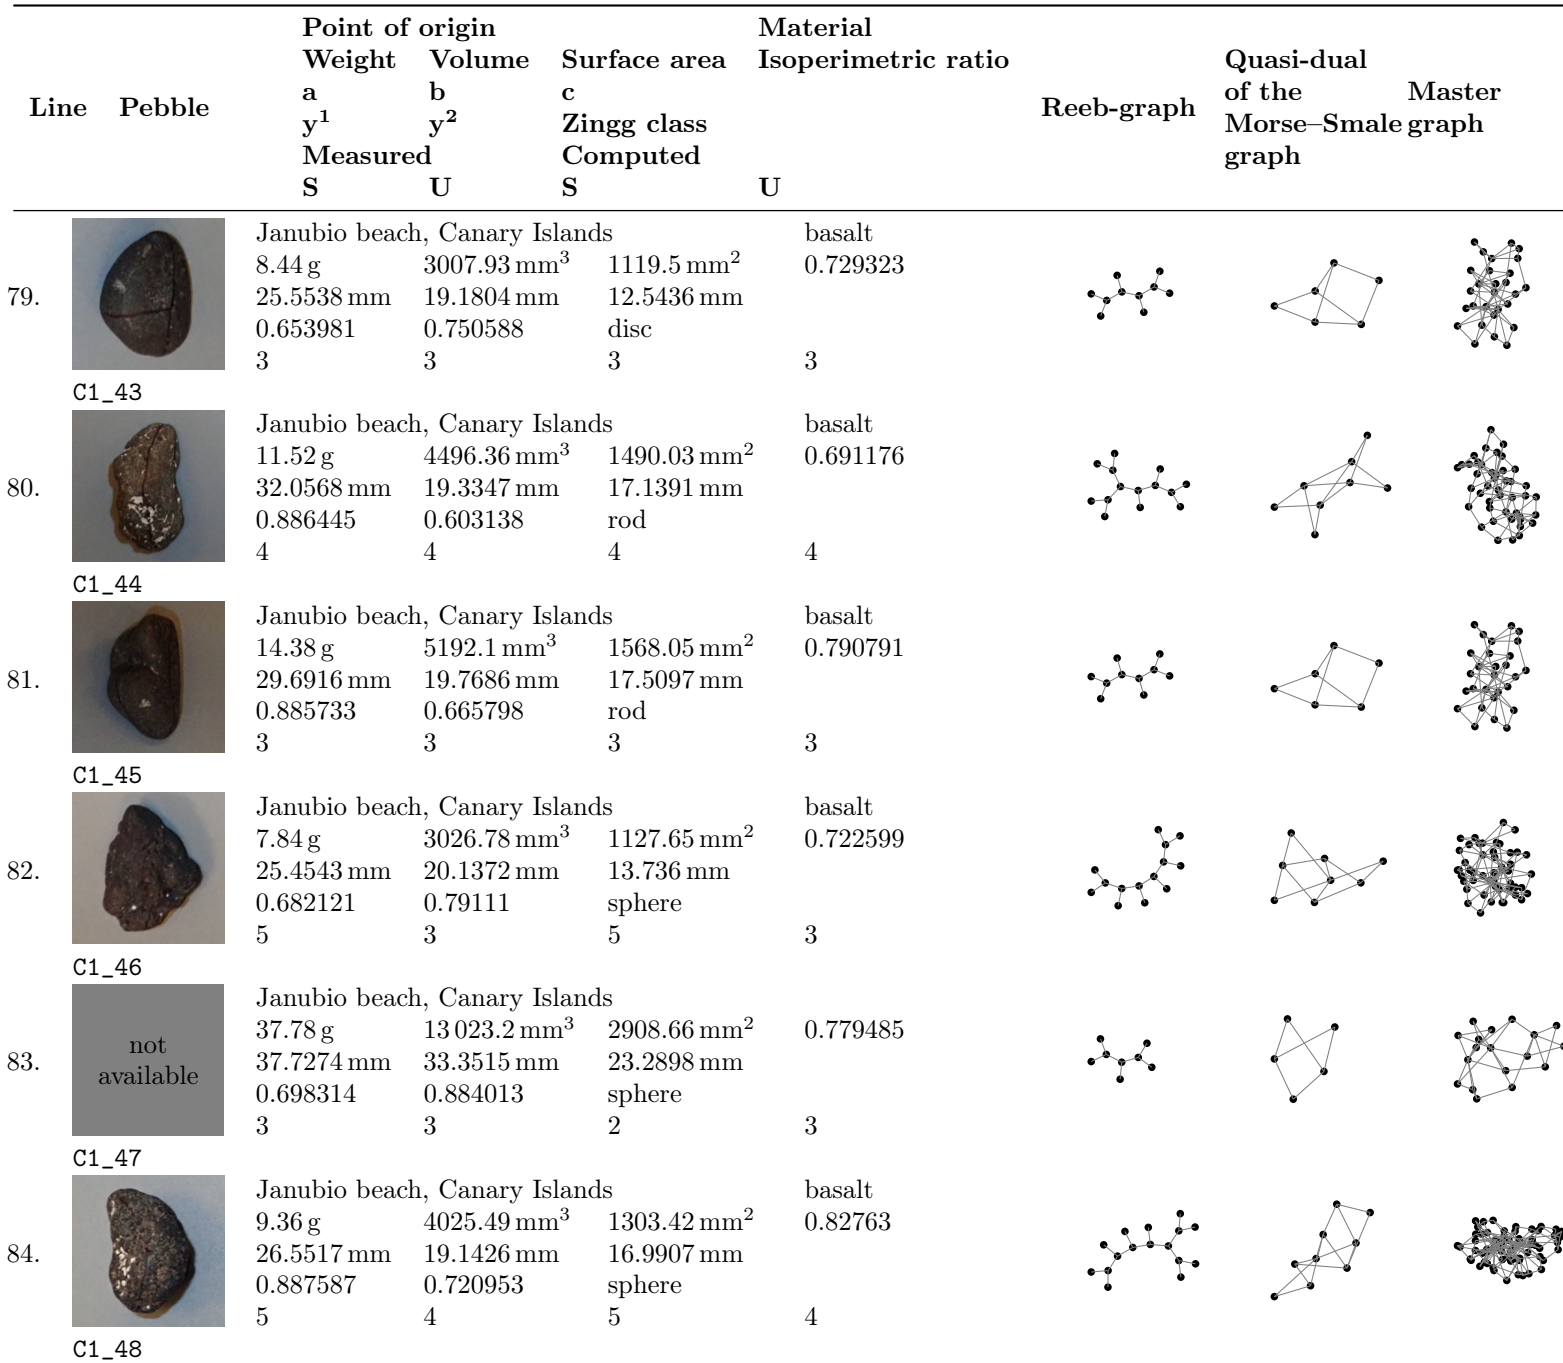 | Janubio beach, Canary Islands   |                          |                              | basalt   | 0.82763             | 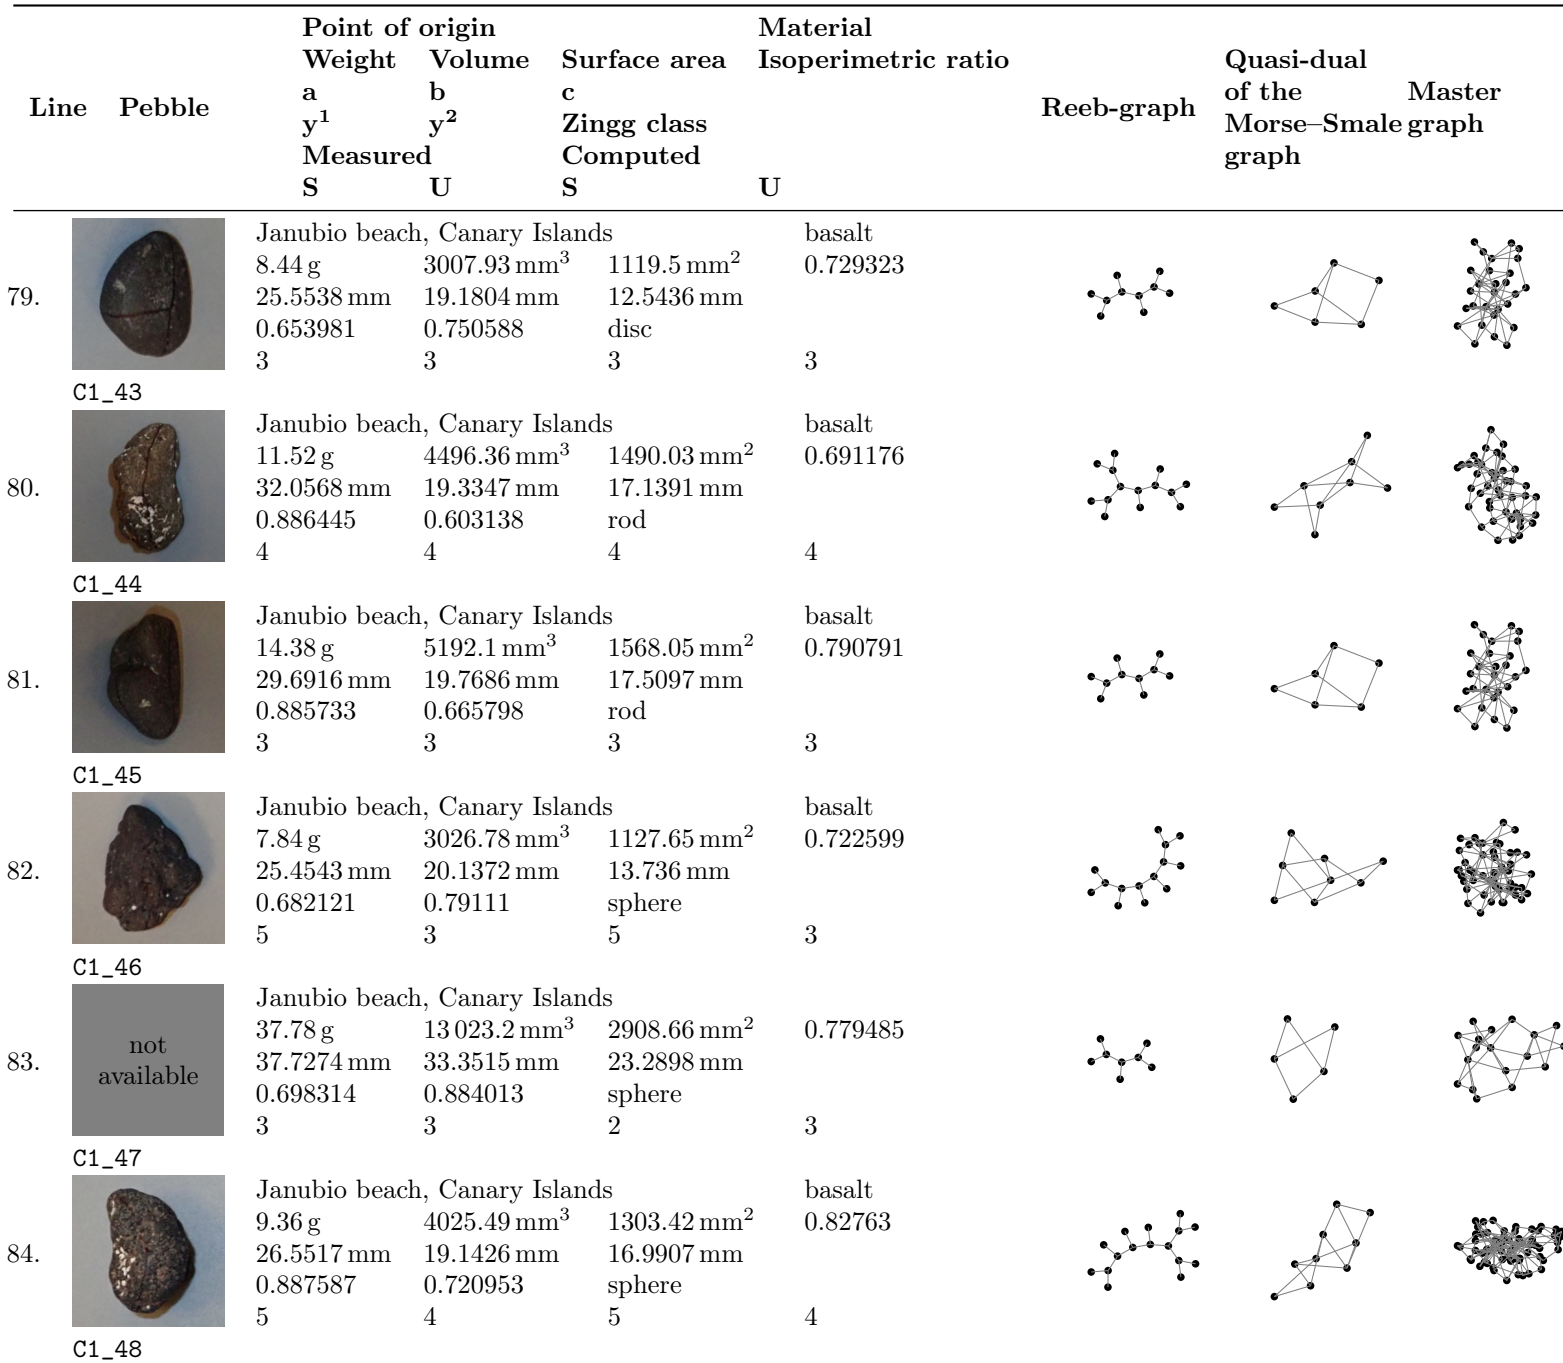 | 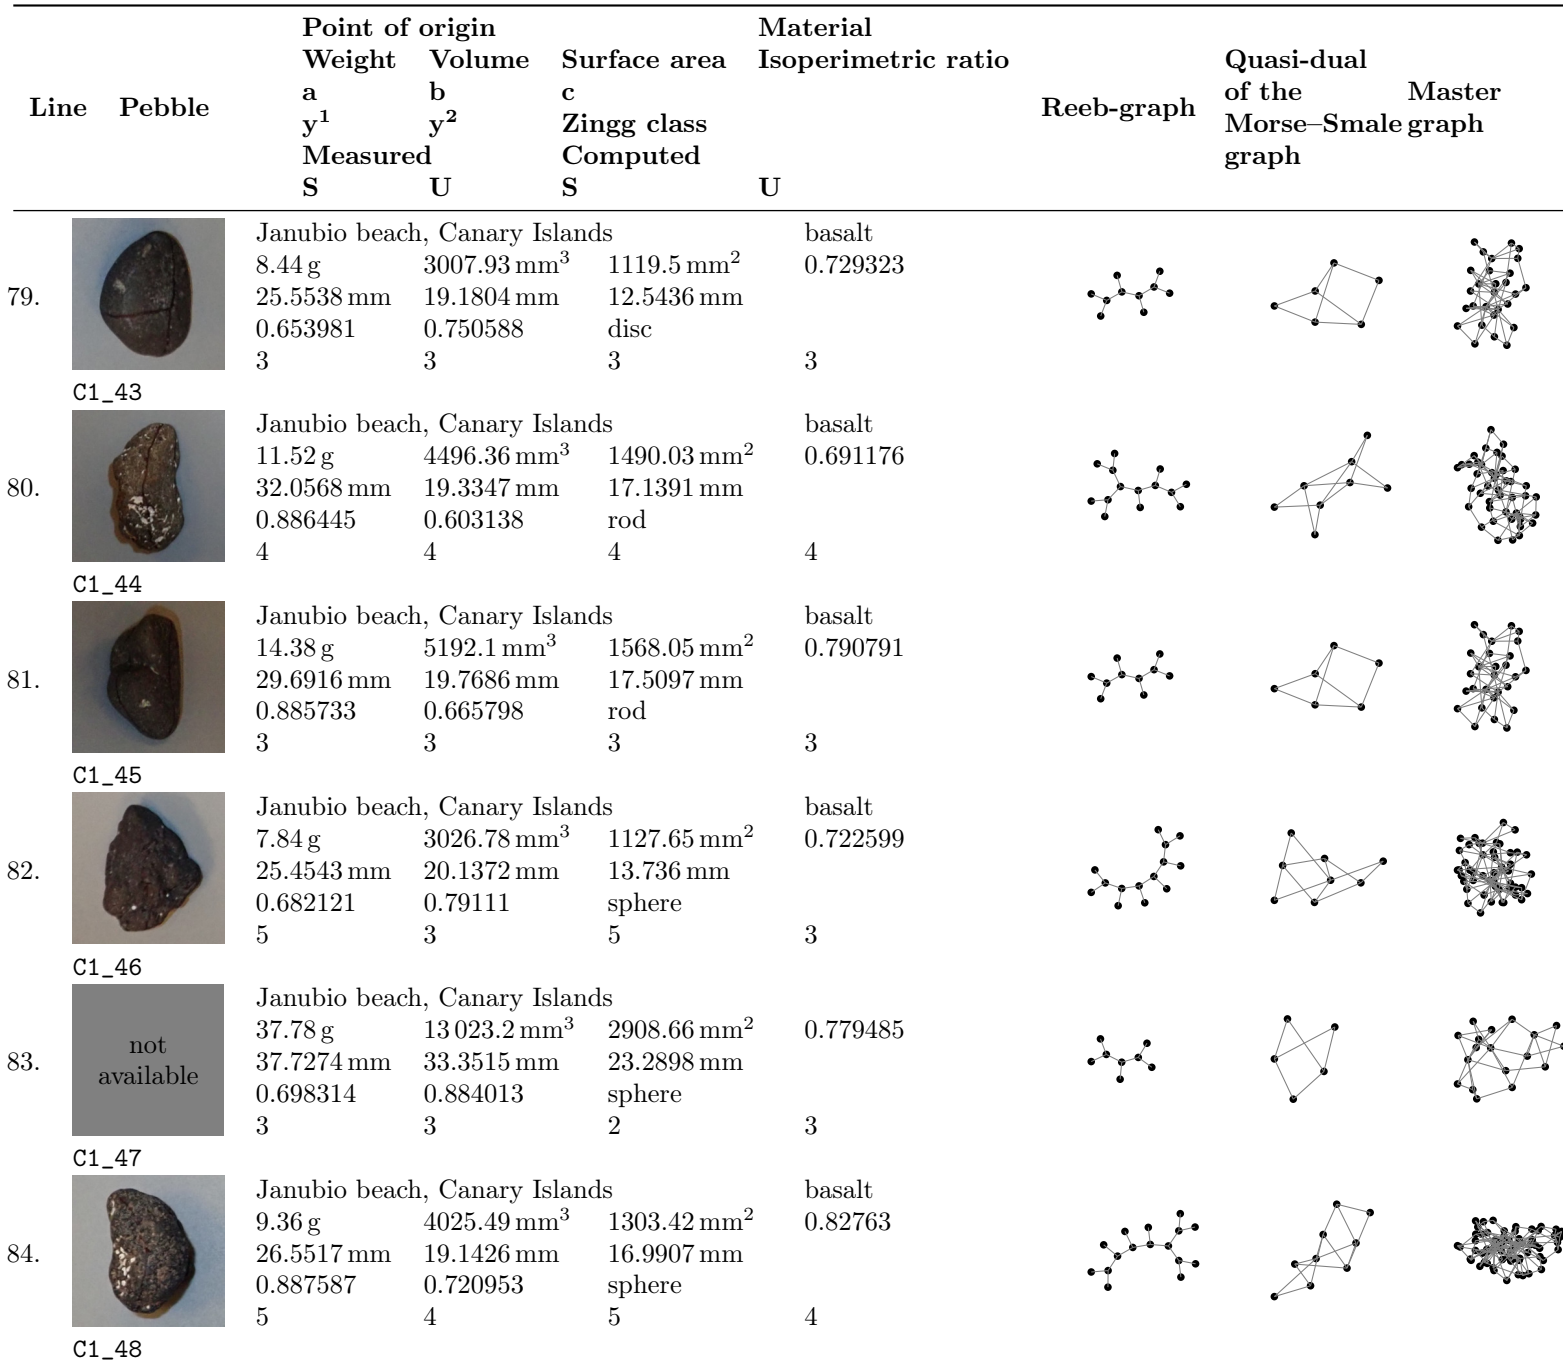 | 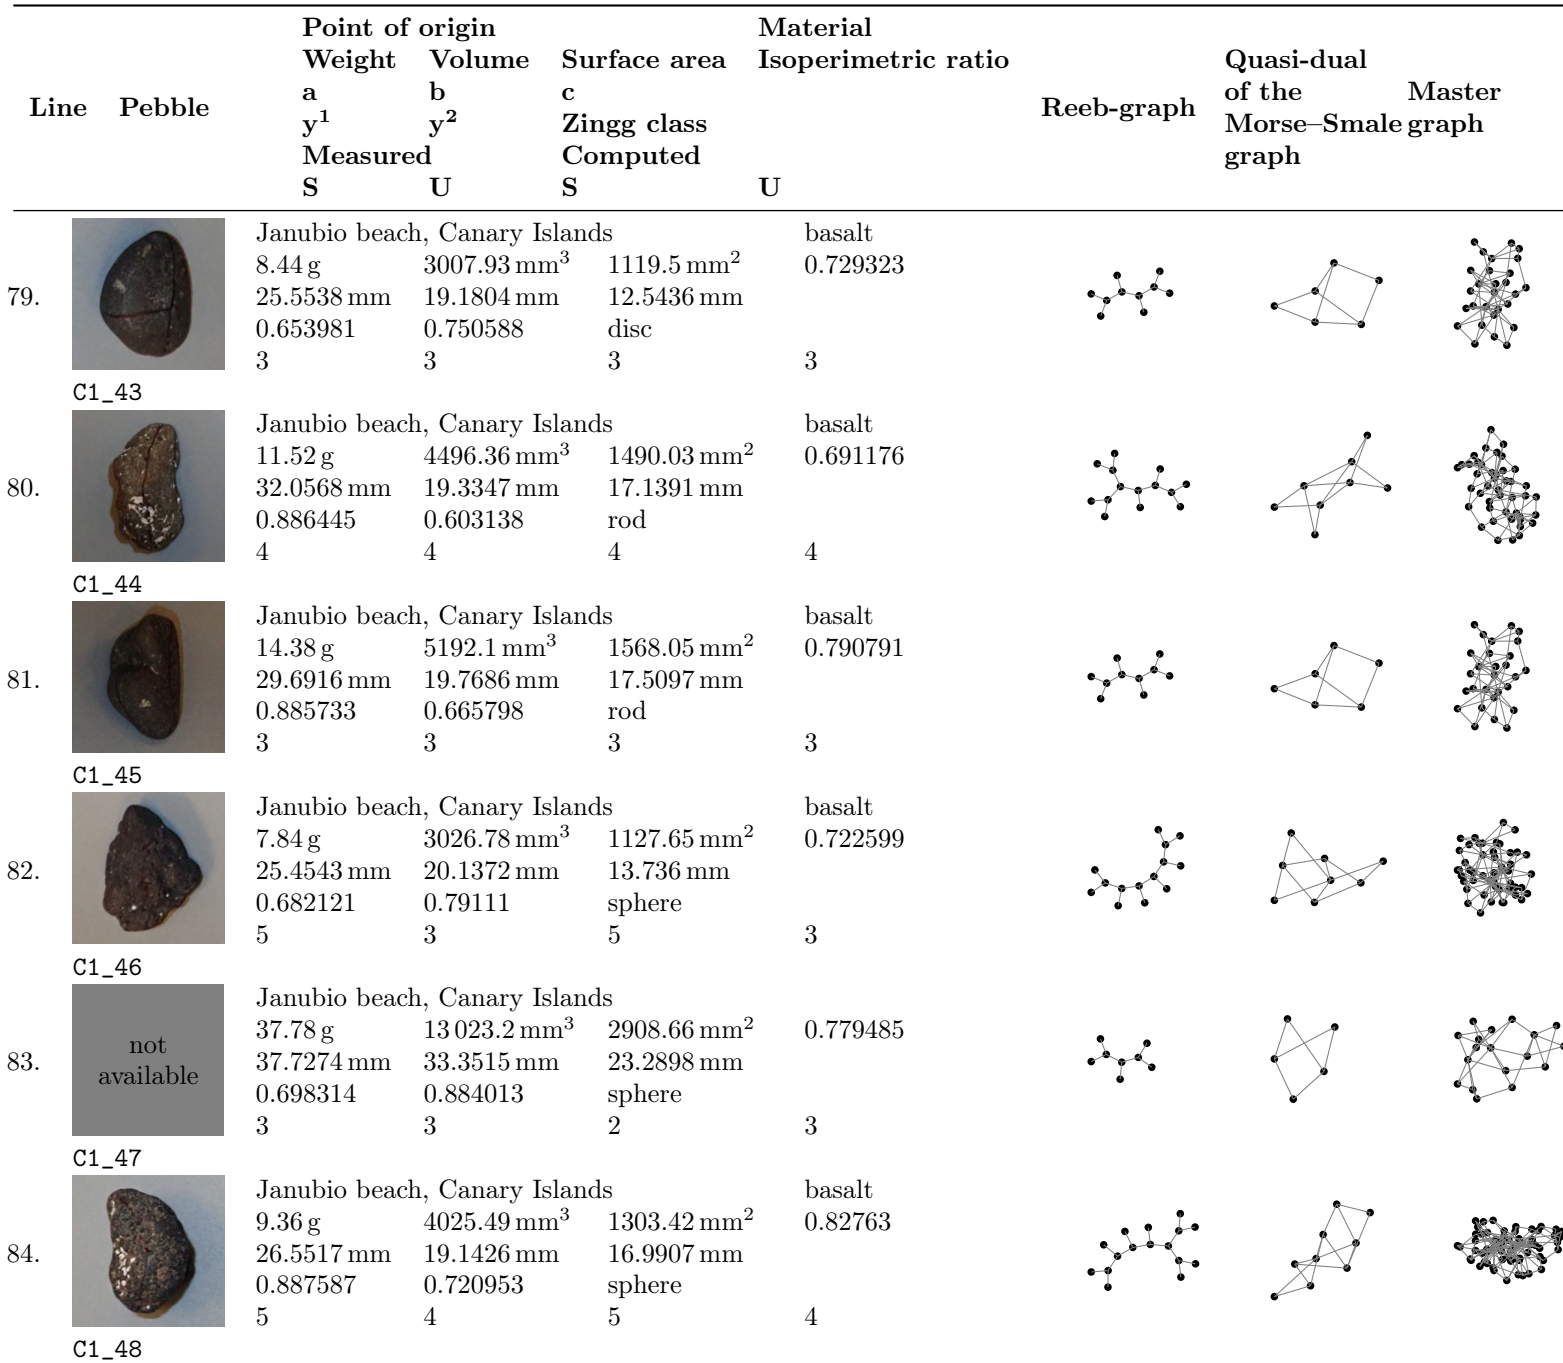 |
|      |                                                                                     | 9.36 g                          | 4025.49 mm <sup>3</sup>  | 1303.42 mm <sup>2</sup>      |          |                     |                                                                                       |                                                                                       |                                                                                       |
|      |                                                                                     | 26.5517 mm                      | 19.1426 mm               | 16.9907 mm                   |          |                     |                                                                                       |                                                                                       |                                                                                       |
|      |                                                                                     | 0.887587                        | 0.720953                 | sphere                       |          |                     |                                                                                       |                                                                                       |                                                                                       |
|      |                                                                                     | 5                               | 4                        | 5                            |          |                     |                                                                                       |                                                                                       |                                                                                       |
|      | C1_48                                                                               |                                 |                          |                              |          |                     |                                                                                       |                                                                                       |                                                                                       |

| Line | Pebble                                                                              | Point of origin                  |                          |                         | Material  | Isoperimetric ratio                                                                   | Reeb-graph                                                                            | Quasi-dual<br>of the<br>Morse–Smale<br>graph                                          | Master<br>graph |
|------|-------------------------------------------------------------------------------------|----------------------------------|--------------------------|-------------------------|-----------|---------------------------------------------------------------------------------------|---------------------------------------------------------------------------------------|---------------------------------------------------------------------------------------|-----------------|
|      |                                                                                     | Weight                           | Volume                   | Surface area            |           |                                                                                       |                                                                                       |                                                                                       |                 |
|      |                                                                                     | a                                | b                        | c                       |           |                                                                                       |                                                                                       |                                                                                       |                 |
|      |                                                                                     | y <sup>1</sup>                   | y <sup>2</sup>           | Zingg class             |           |                                                                                       |                                                                                       |                                                                                       |                 |
|      |                                                                                     | Measured                         | U                        | Computed                |           |                                                                                       |                                                                                       |                                                                                       |                 |
| S    |                                                                                     | S                                | U                        | S                       | U         |                                                                                       |                                                                                       |                                                                                       |                 |
| 85.  | 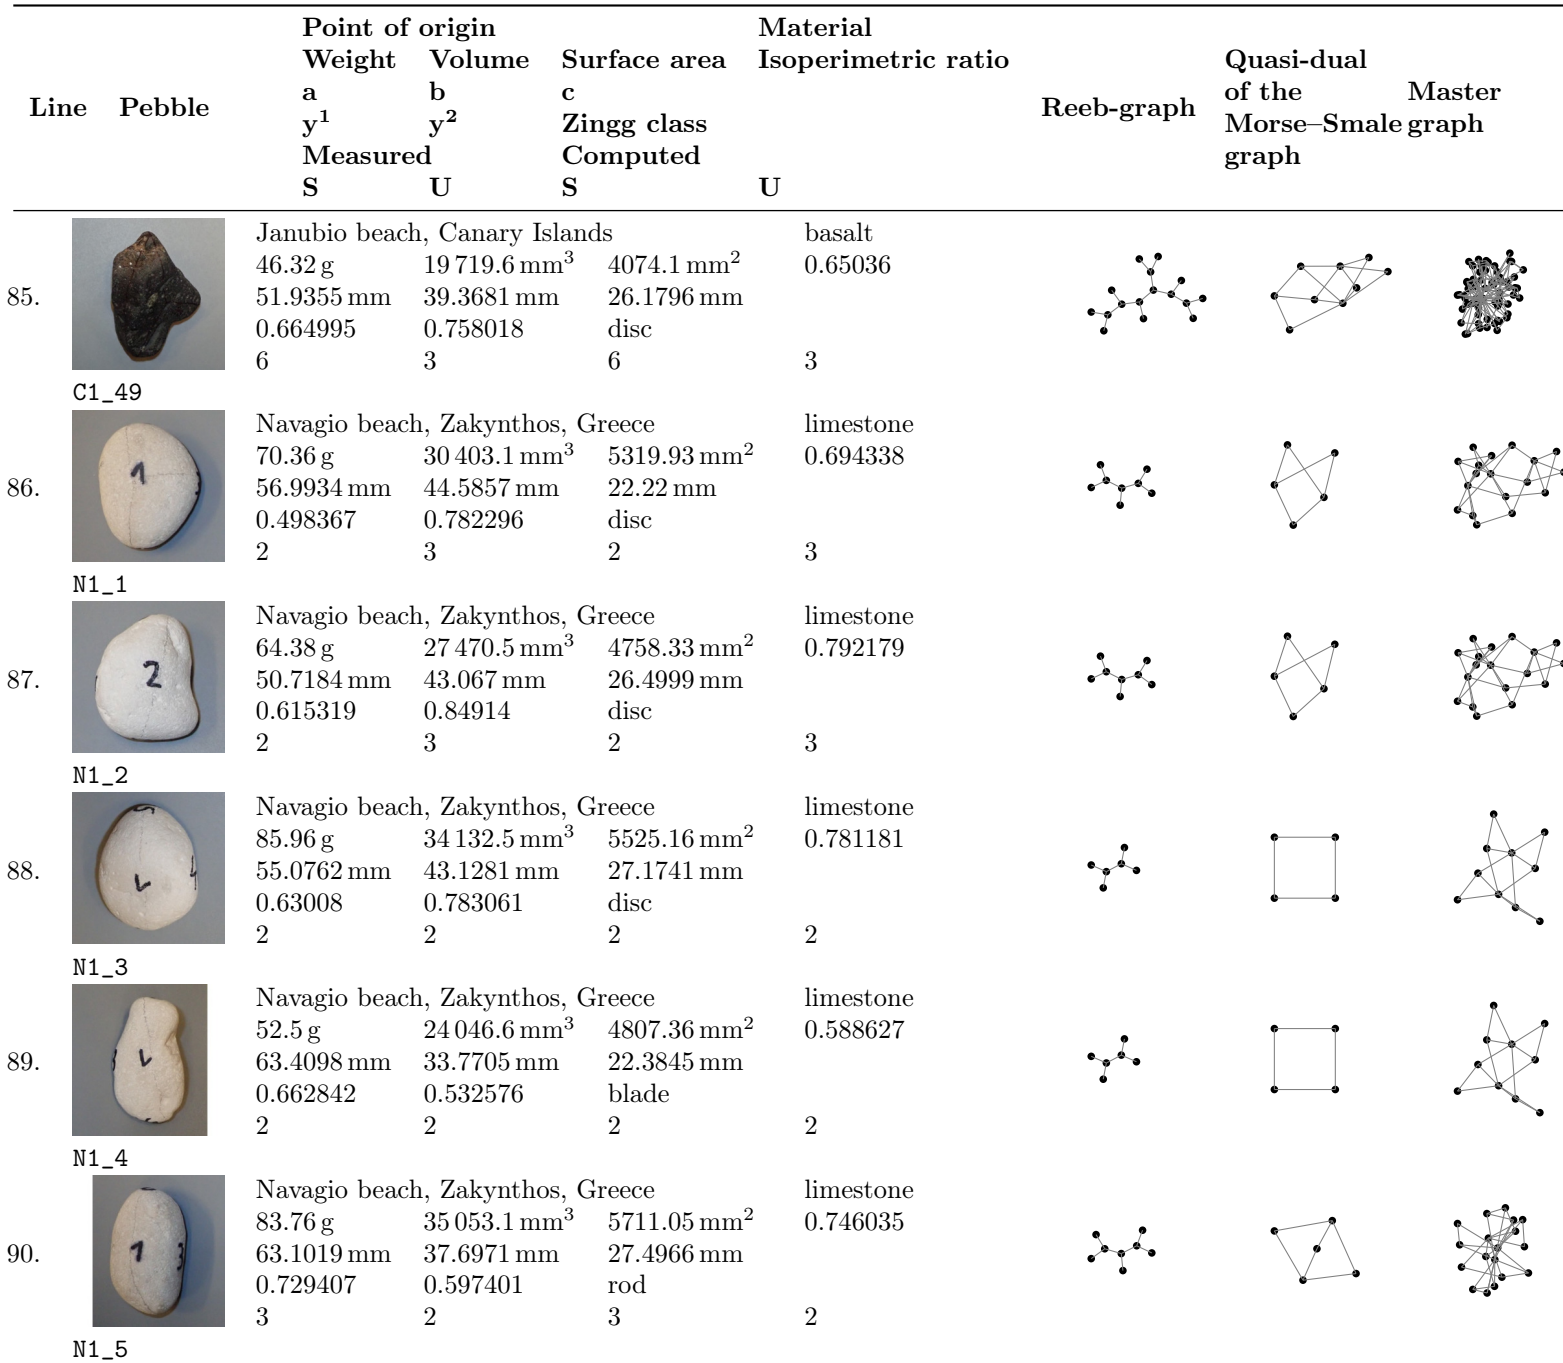   | Janubio beach, Canary Islands    |                          |                         | basalt    | 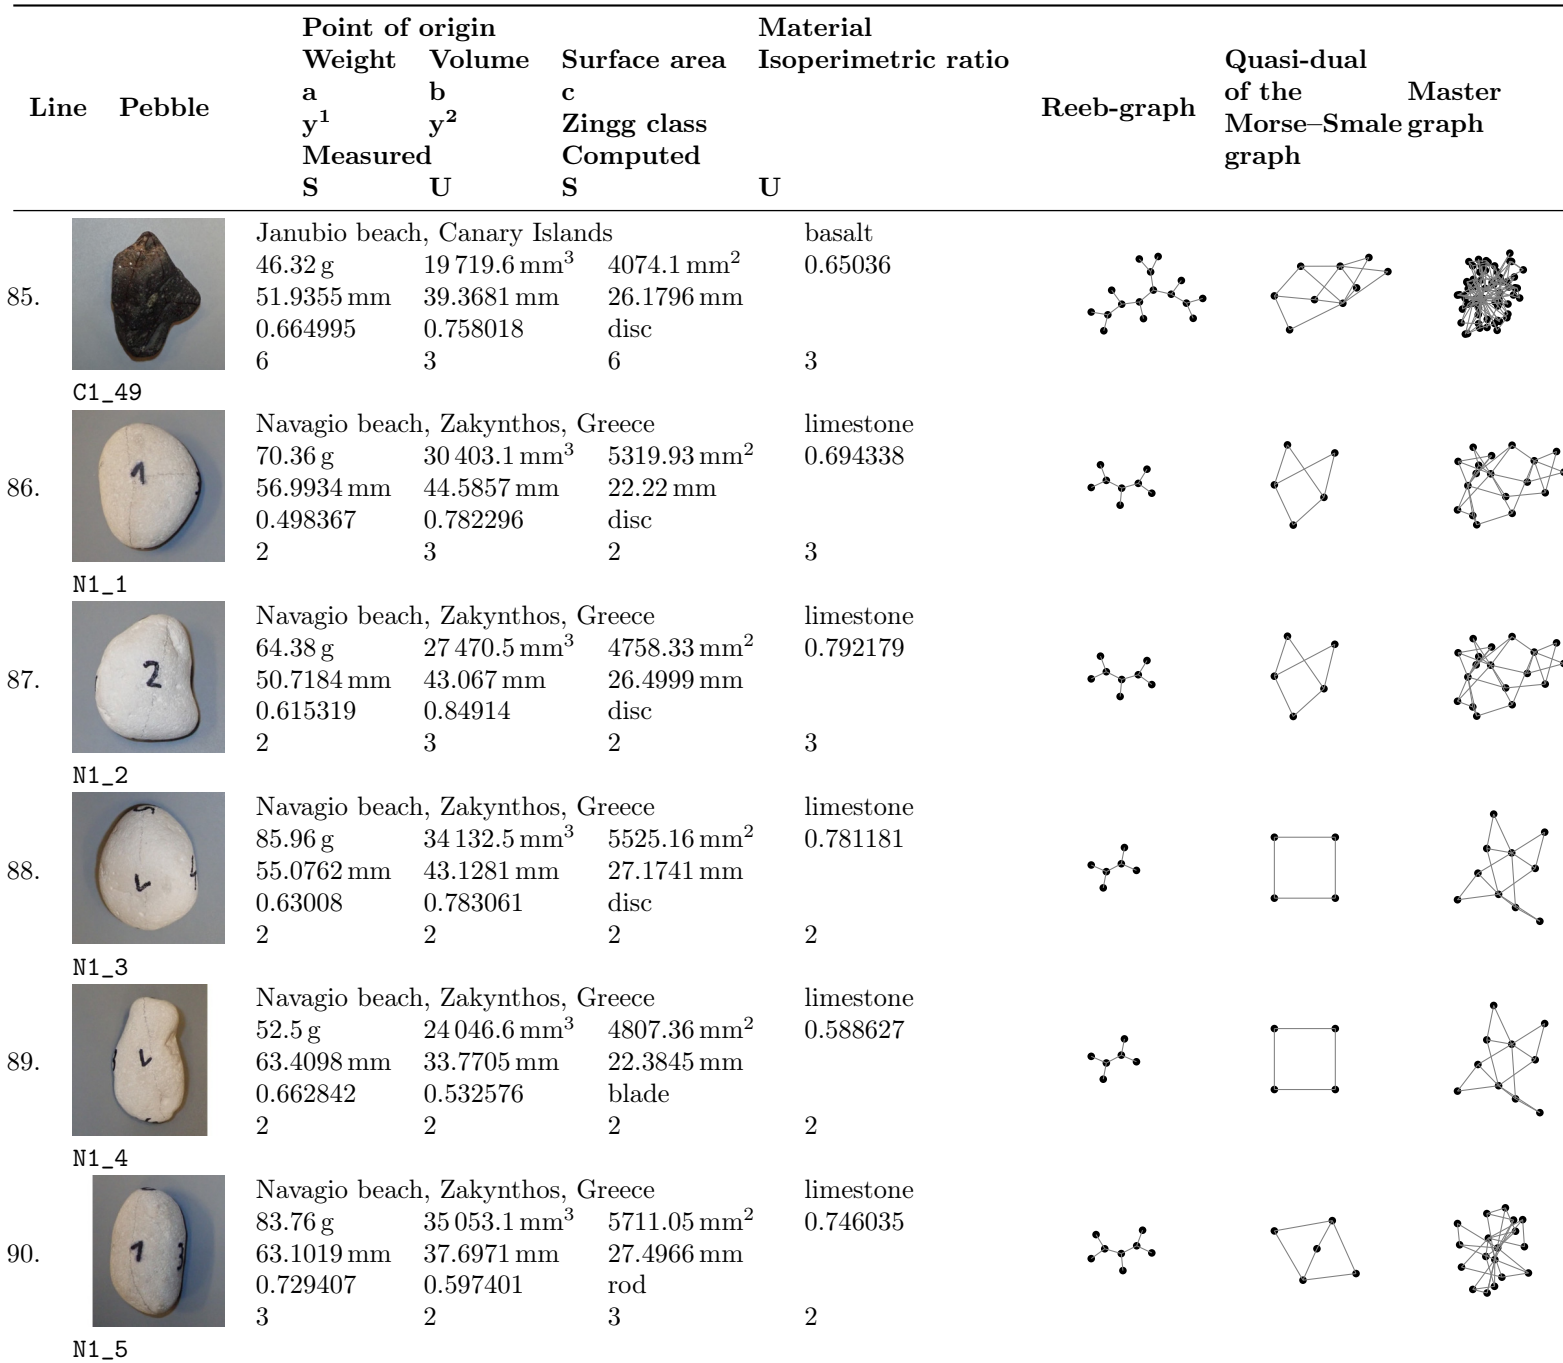   | 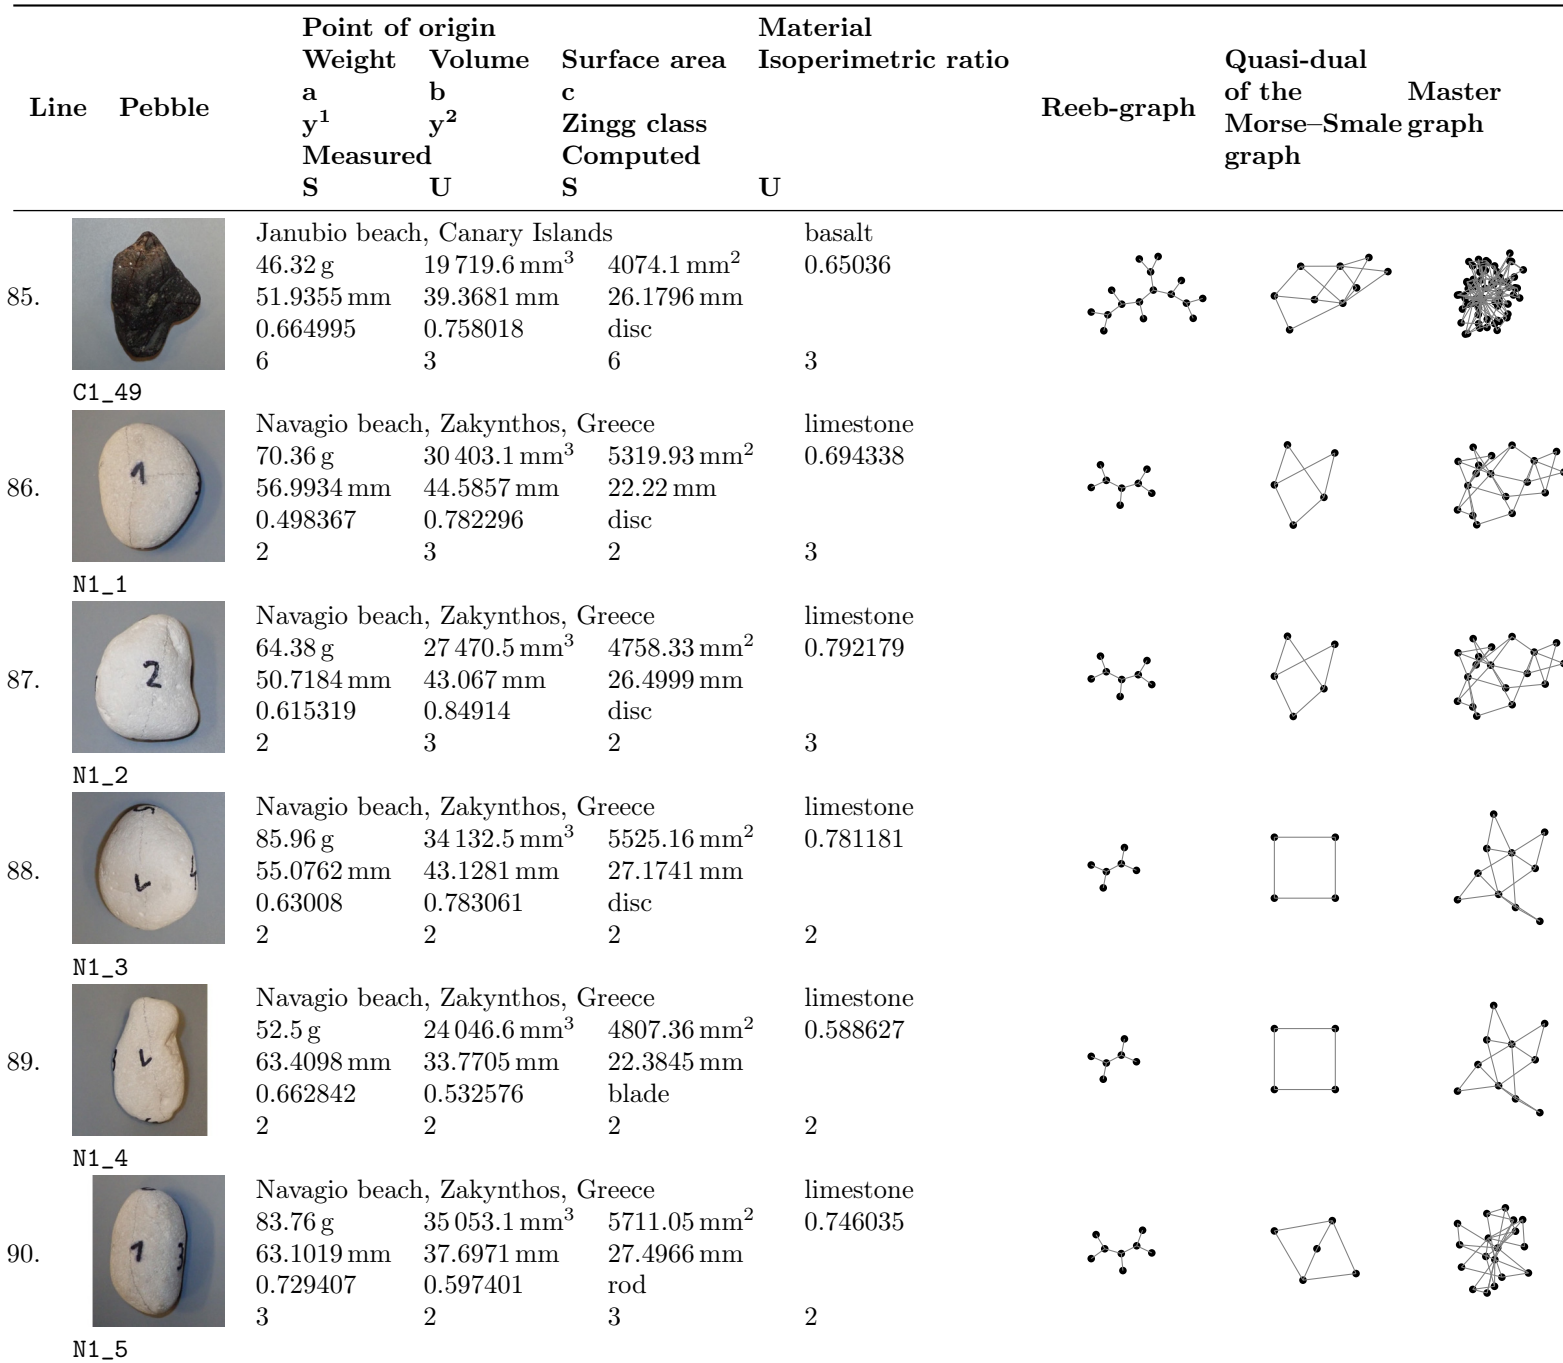   | 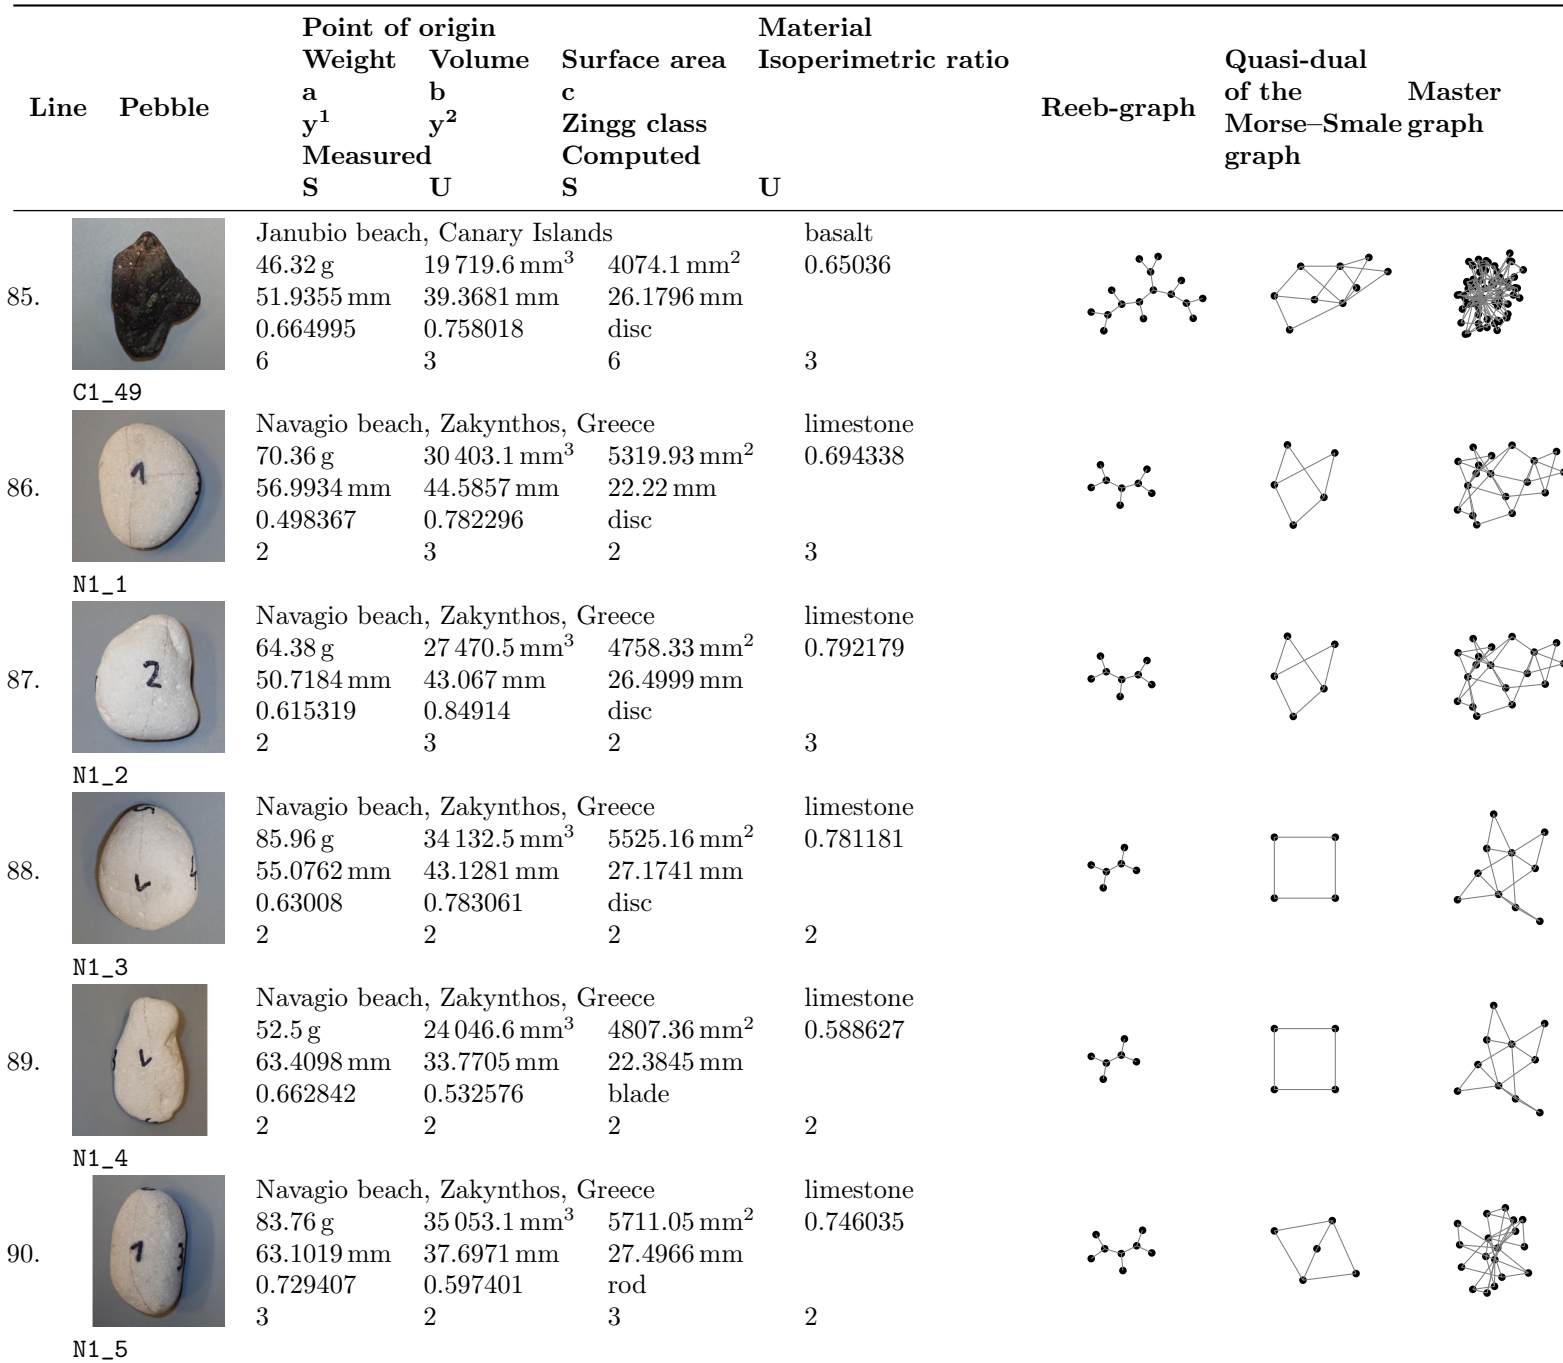   |                 |
|      |                                                                                     | 46.32 g                          | 19 719.6 mm <sup>3</sup> | 4074.1 mm <sup>2</sup>  | 0.65036   |                                                                                       |                                                                                       |                                                                                       |                 |
|      |                                                                                     | 51.9355 mm                       | 39.3681 mm               | 26.1796 mm              |           |                                                                                       |                                                                                       |                                                                                       |                 |
|      |                                                                                     | 0.664995                         | 0.758018                 | disc                    |           |                                                                                       |                                                                                       |                                                                                       |                 |
|      |                                                                                     | 6                                | 3                        | 6                       | 3         |                                                                                       |                                                                                       |                                                                                       |                 |
| 86.  | 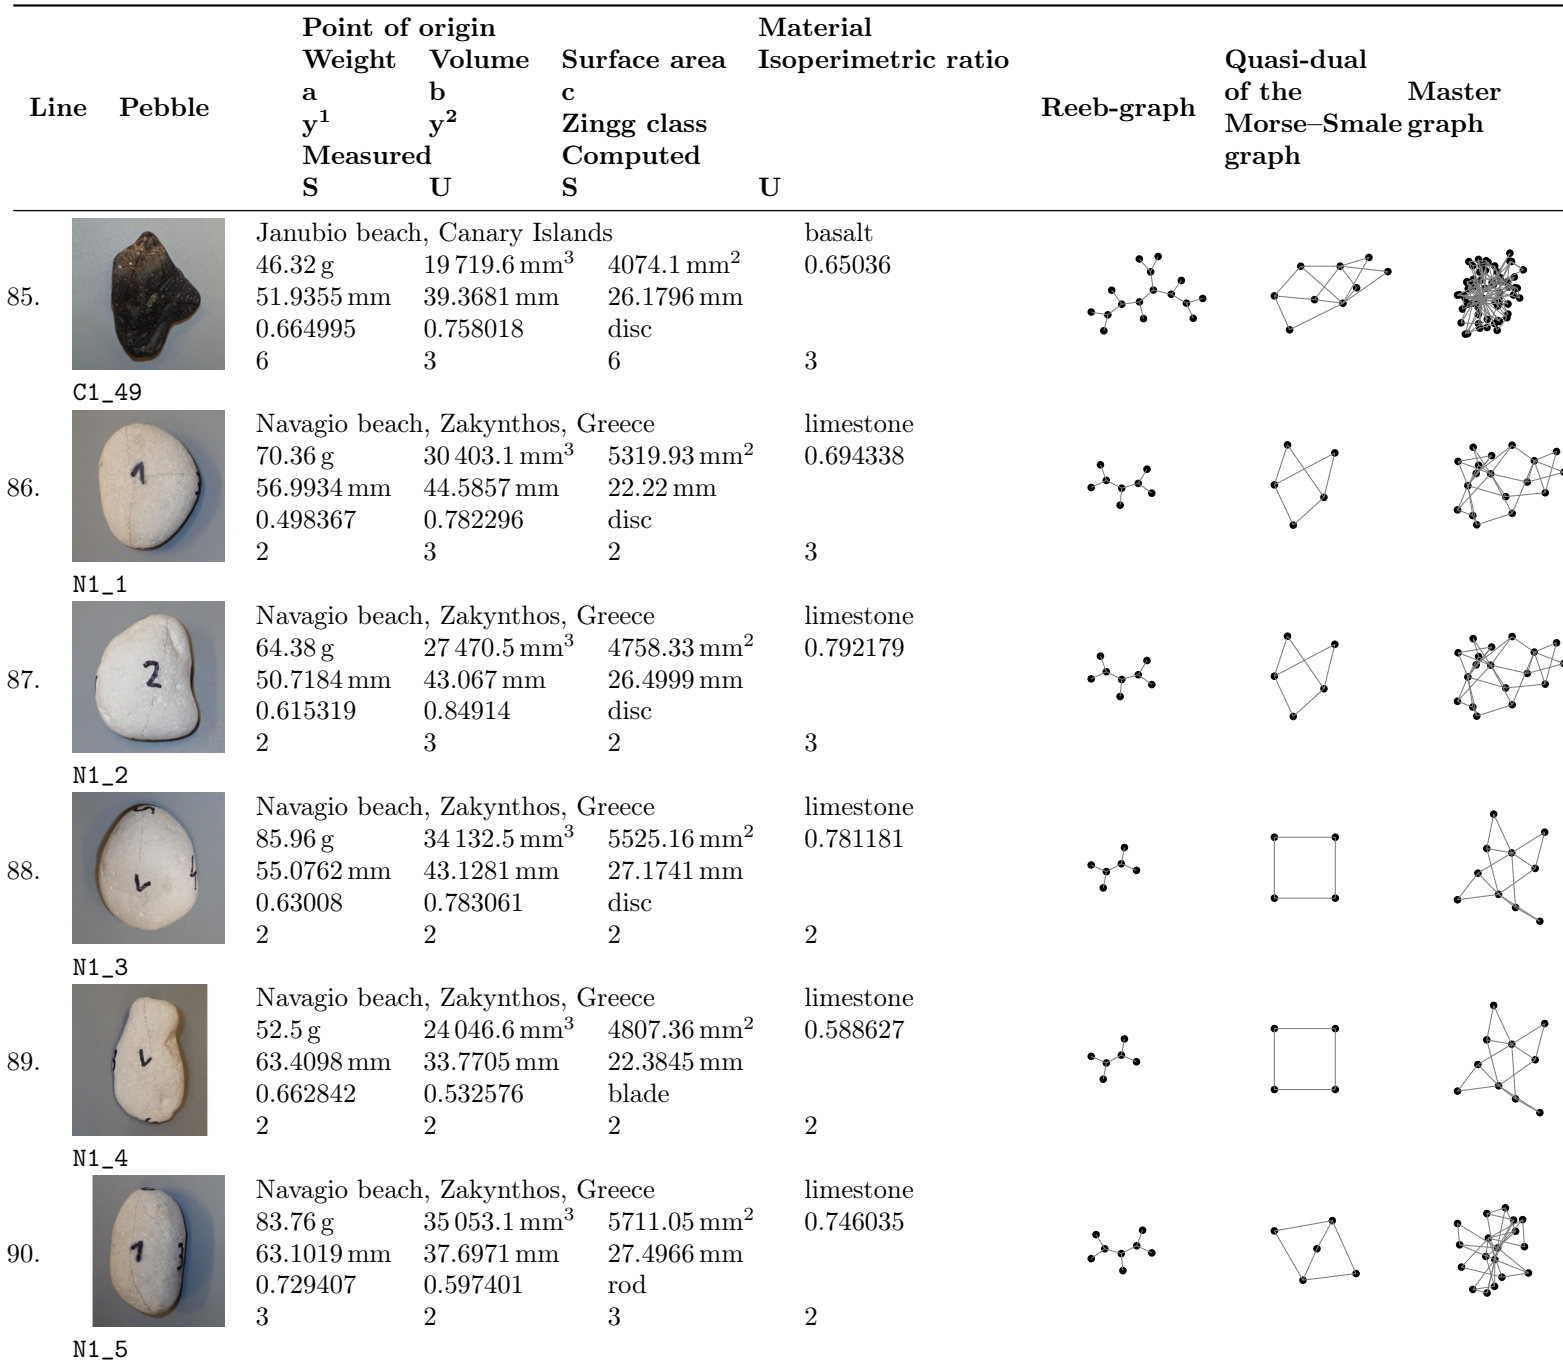   | Navagio beach, Zakynthos, Greece |                          |                         | limestone | 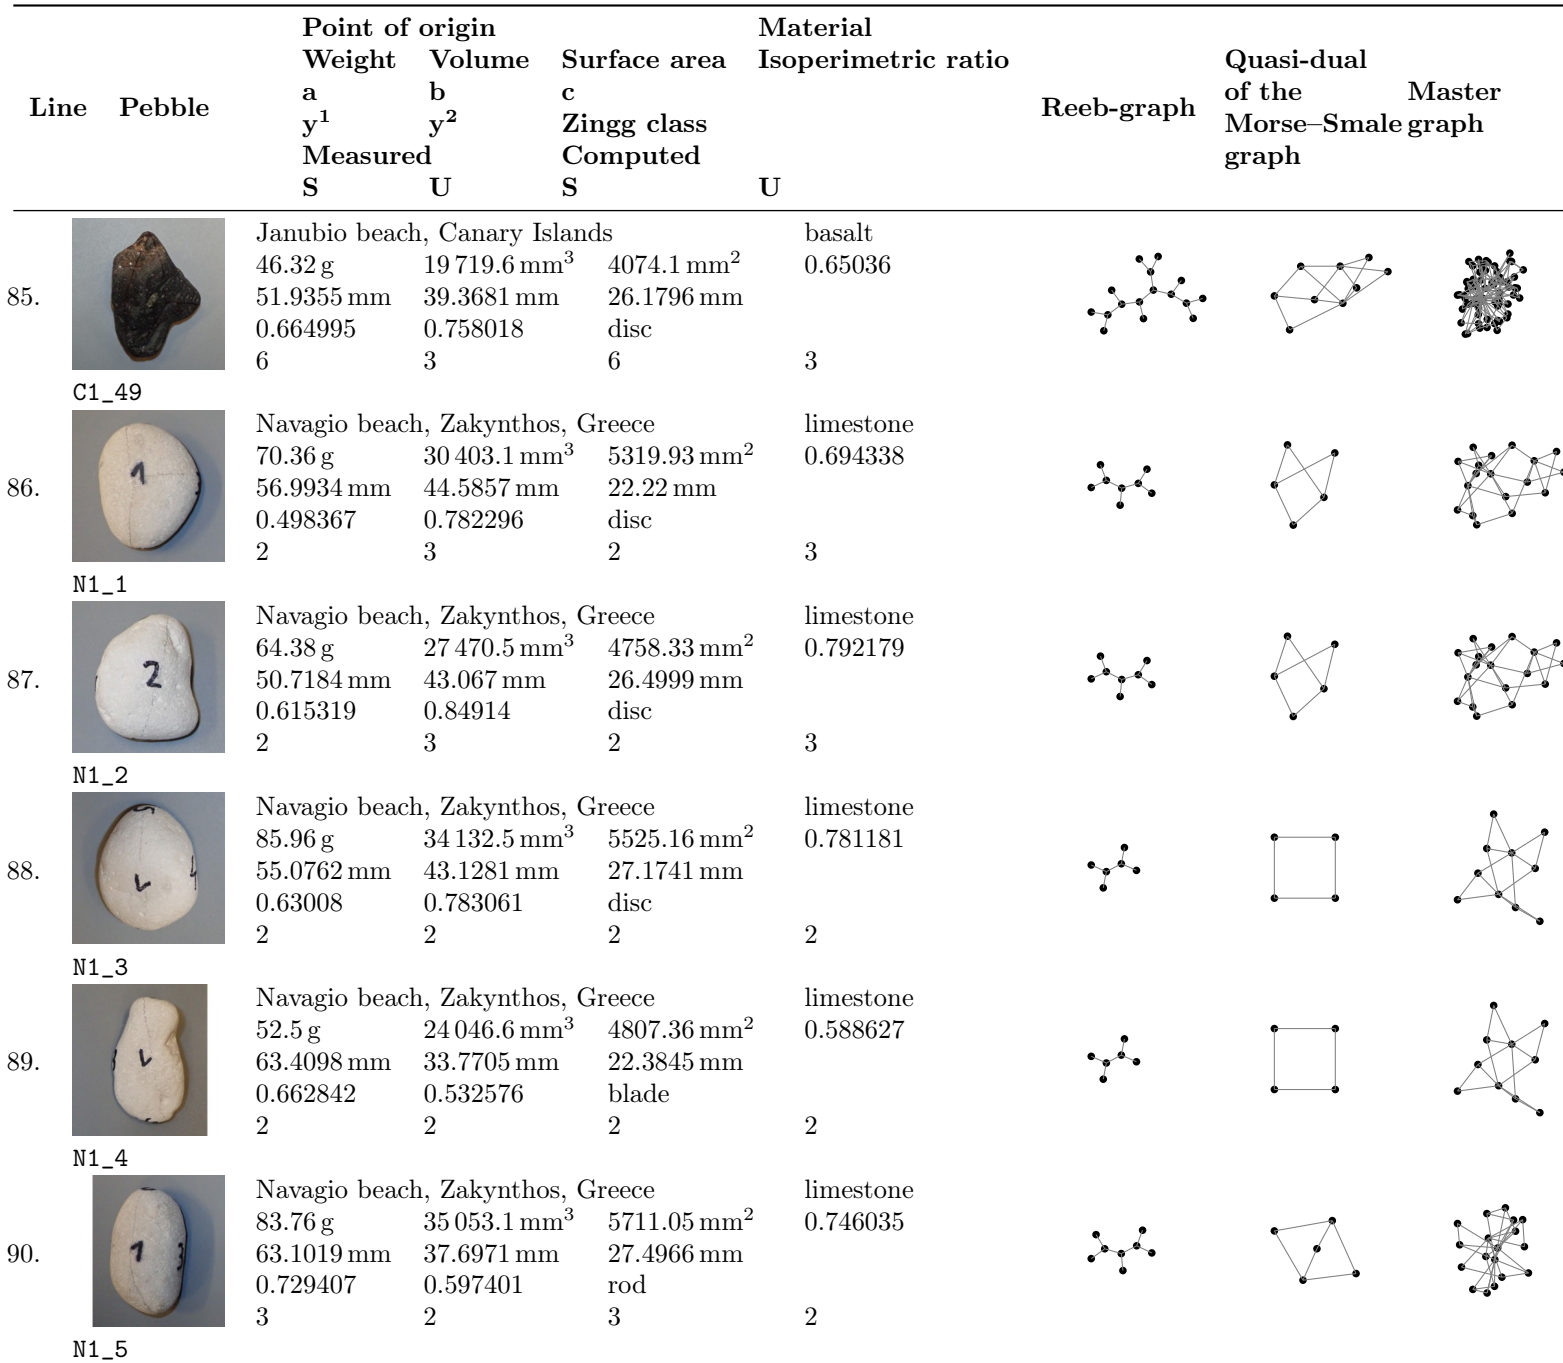   | 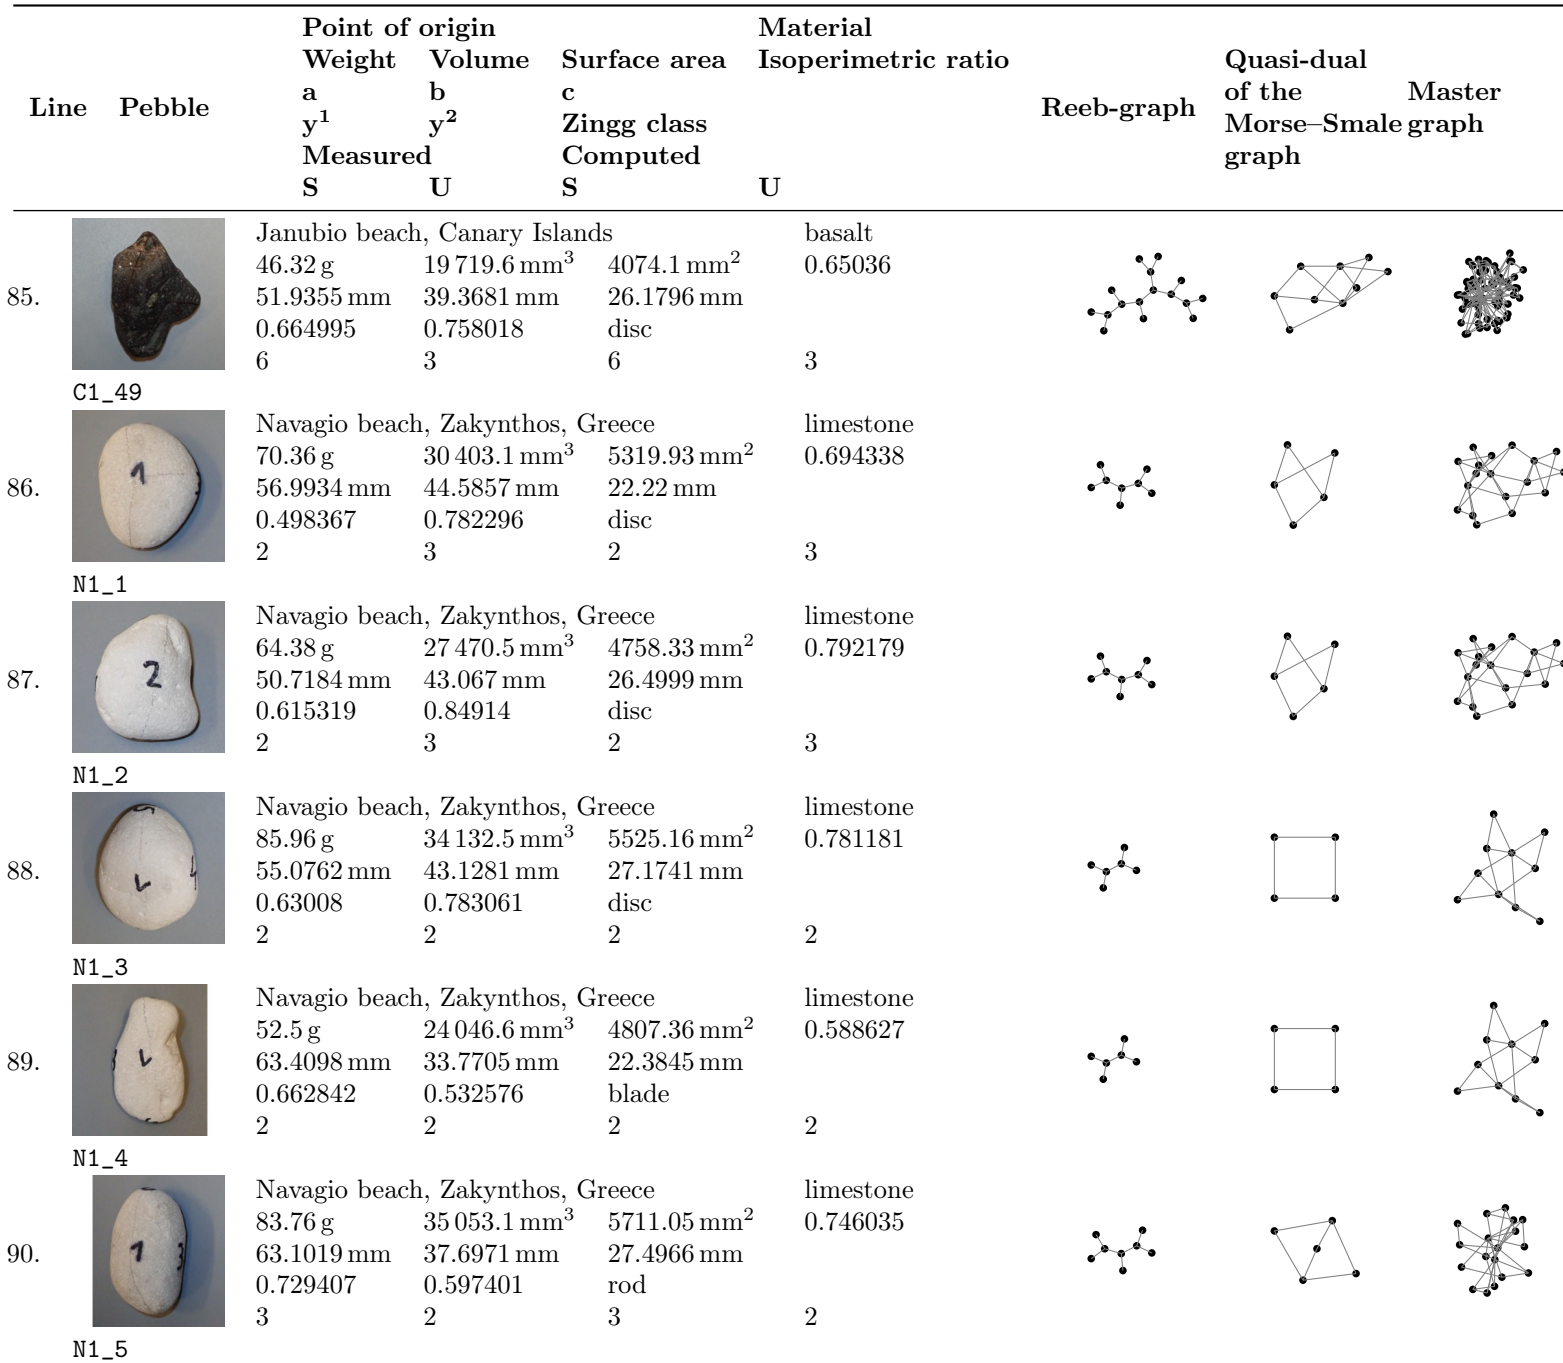   | 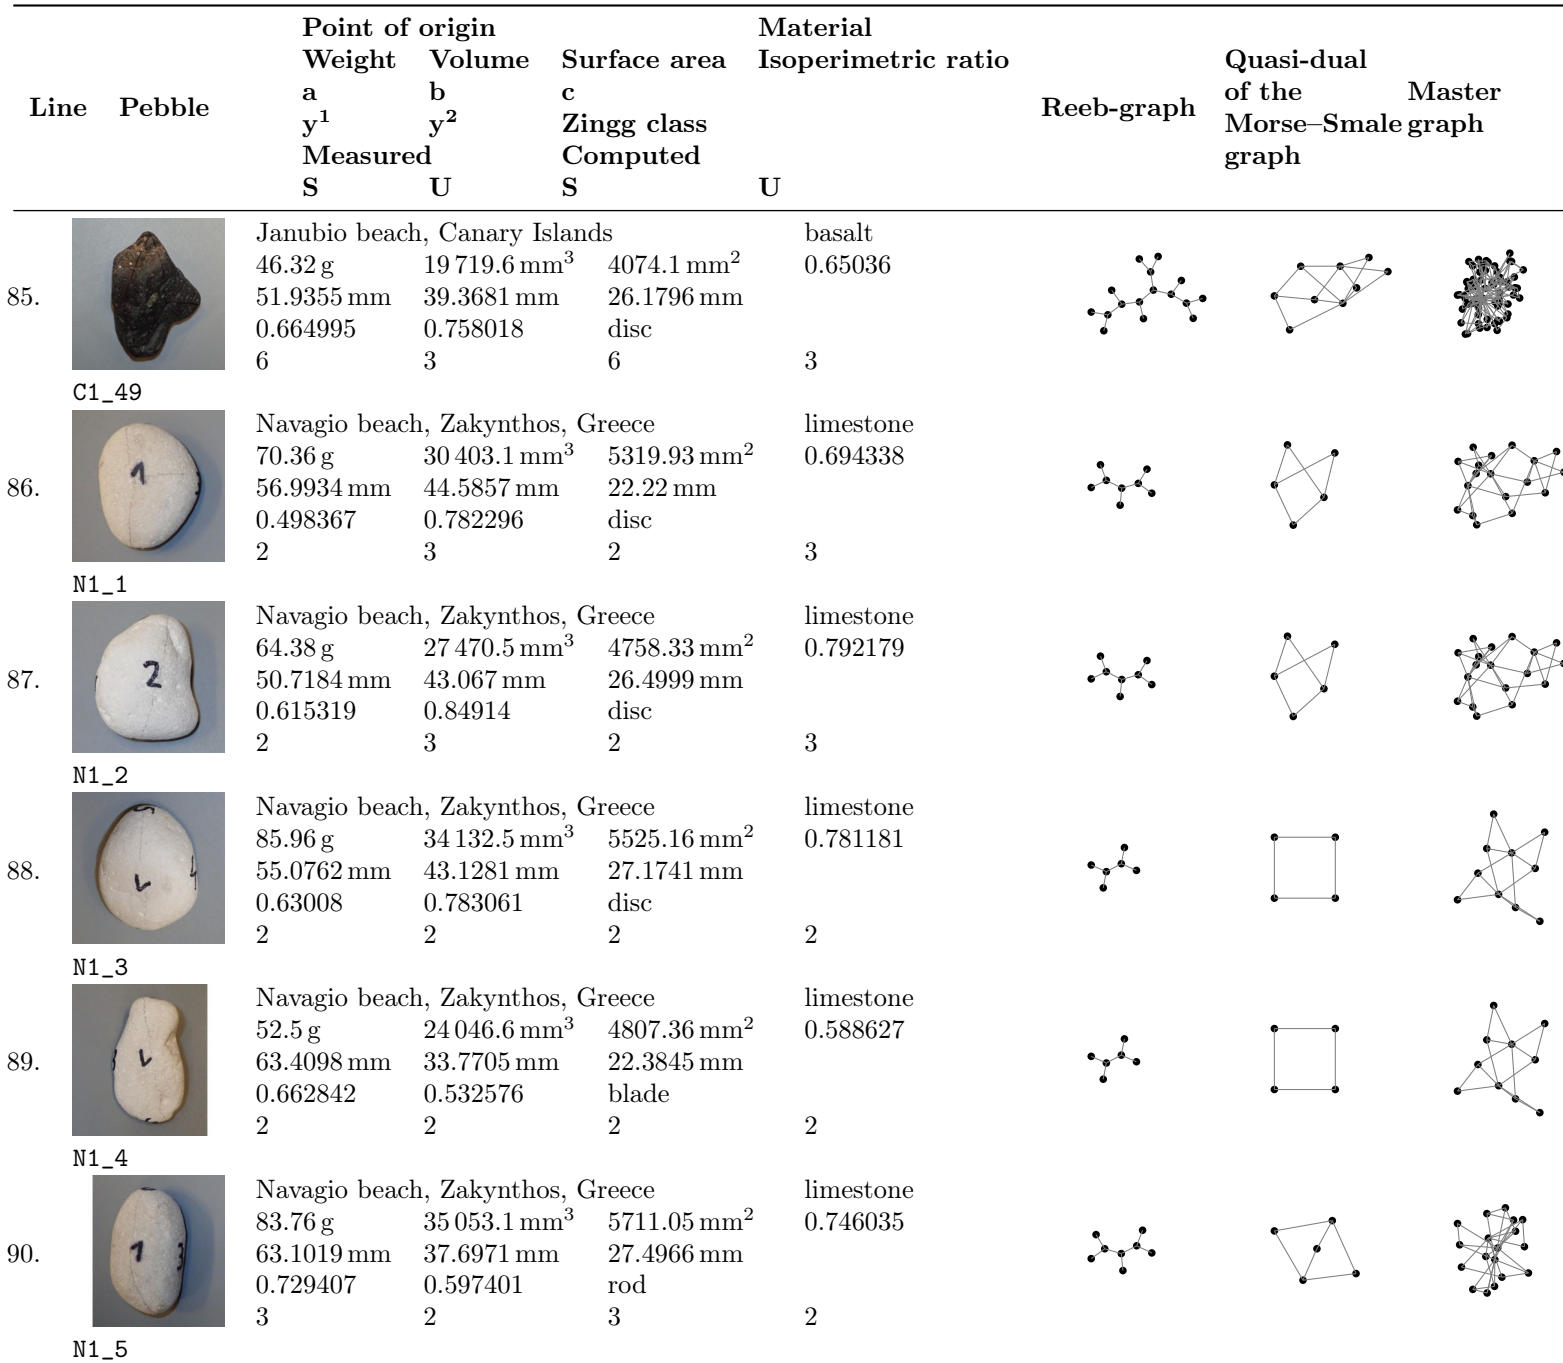   |                 |
|      |                                                                                     | 70.36 g                          | 30 403.1 mm <sup>3</sup> | 5319.93 mm <sup>2</sup> | 0.694338  |                                                                                       |                                                                                       |                                                                                       |                 |
|      |                                                                                     | 56.9934 mm                       | 44.5857 mm               | 22.22 mm                |           |                                                                                       |                                                                                       |                                                                                       |                 |
|      |                                                                                     | 0.498367                         | 0.782296                 | disc                    |           |                                                                                       |                                                                                       |                                                                                       |                 |
|      |                                                                                     | 2                                | 3                        | 2                       | 3         |                                                                                       |                                                                                       |                                                                                       |                 |
| 87.  | 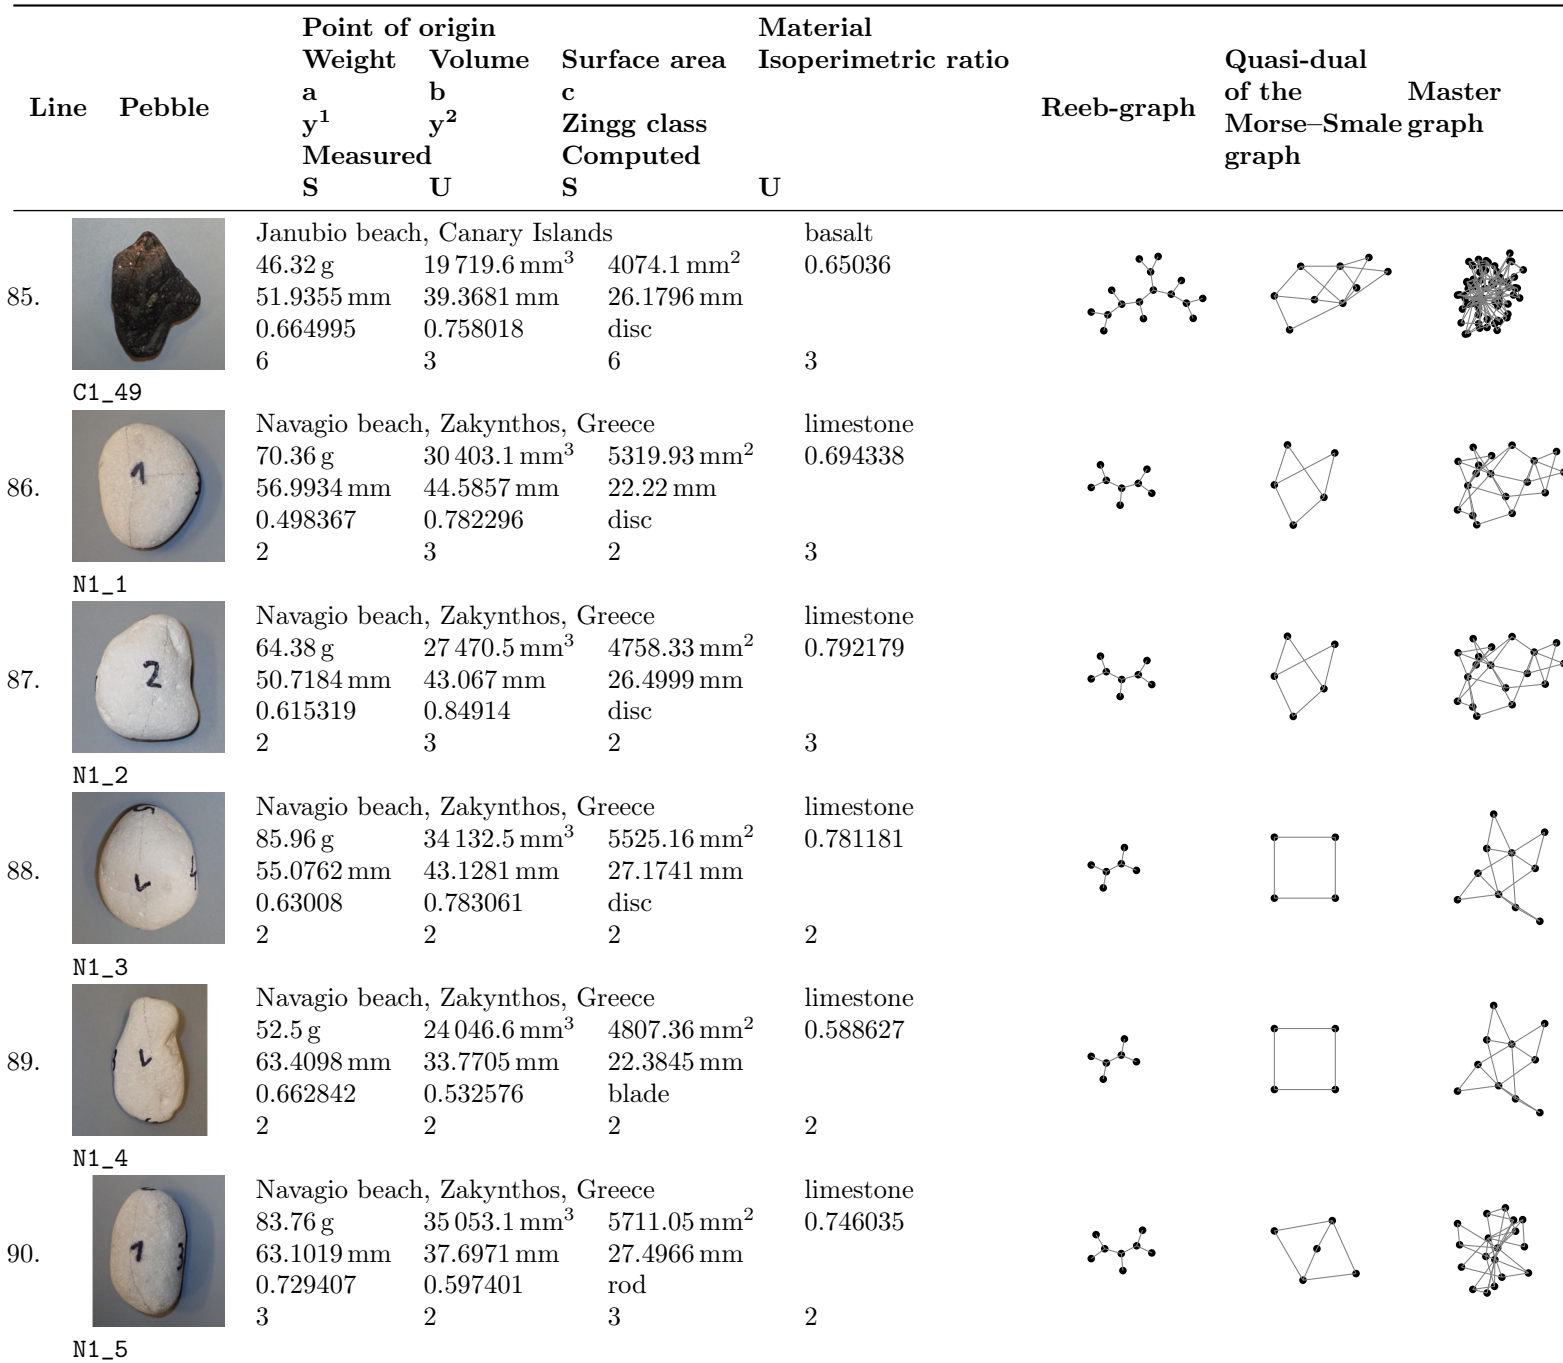   | Navagio beach, Zakynthos, Greece |                          |                         | limestone | 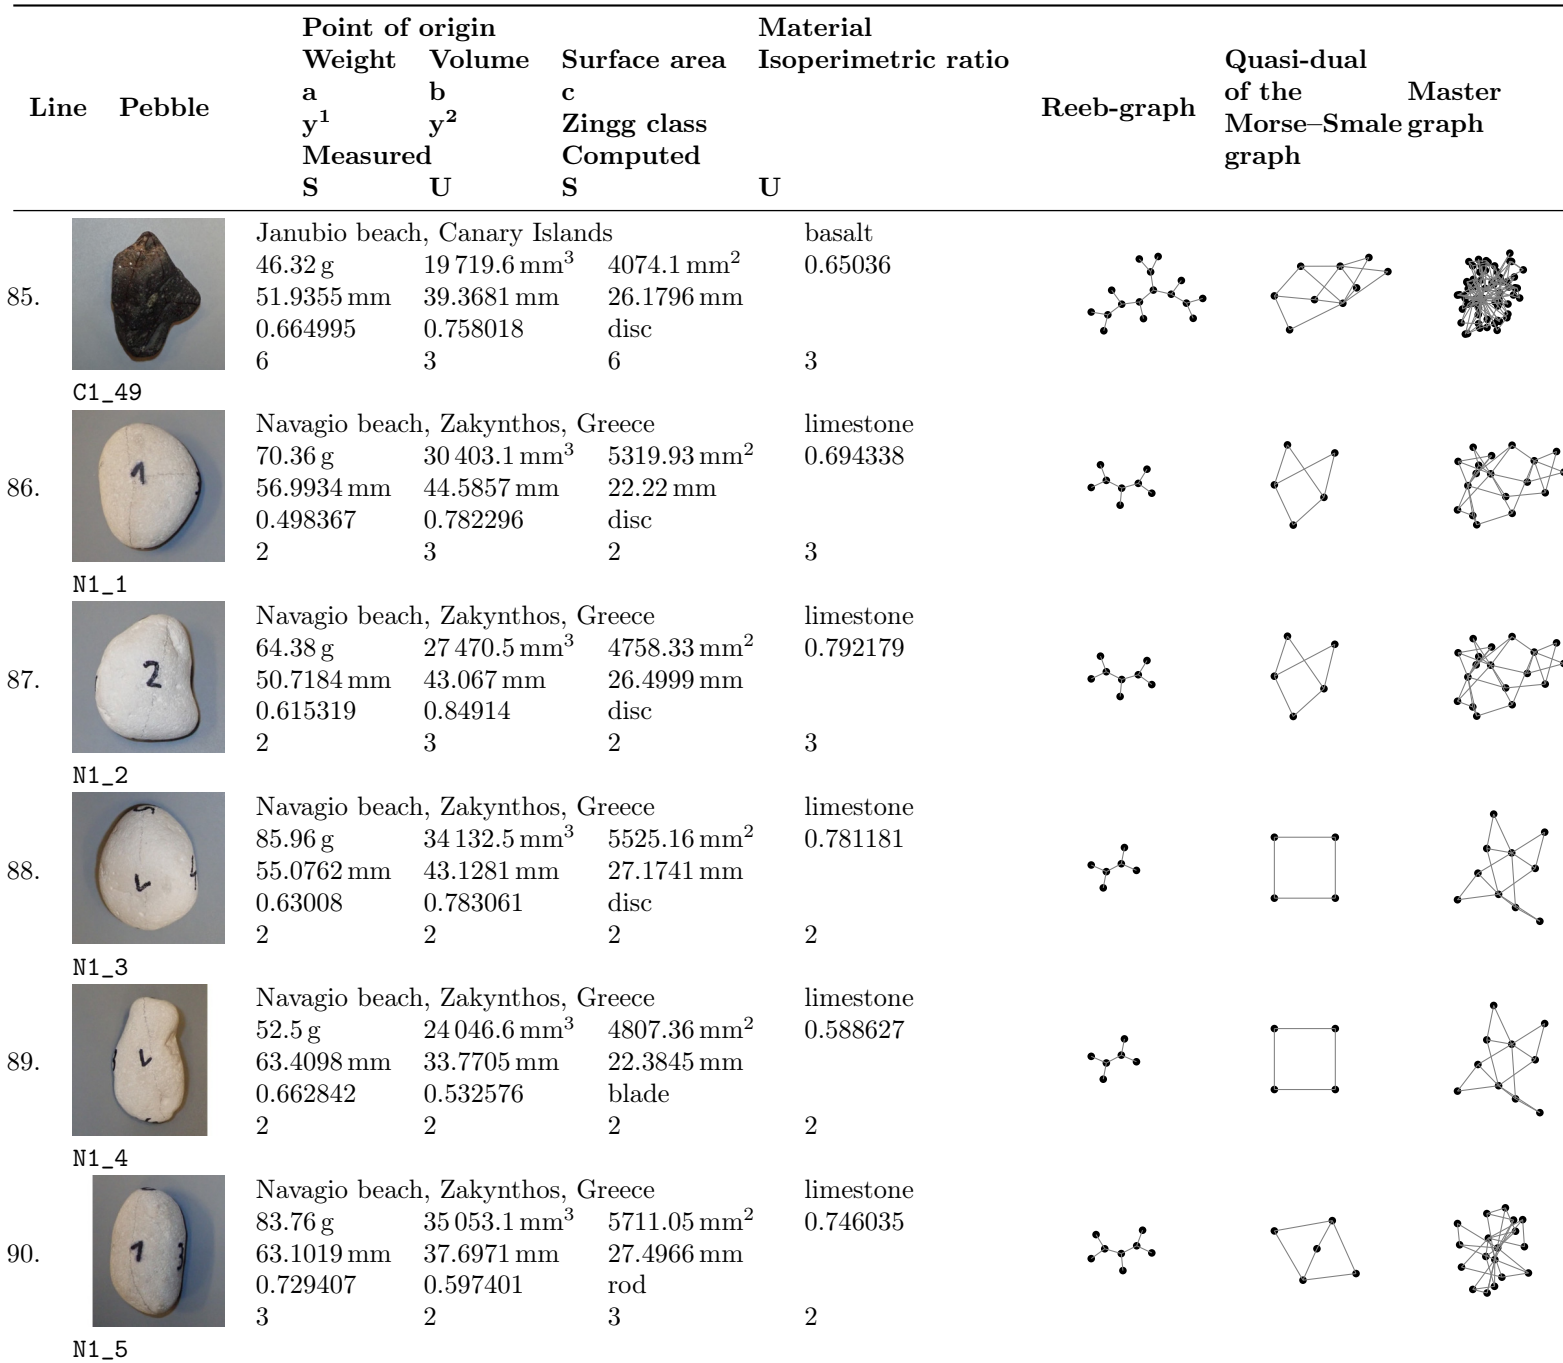   | 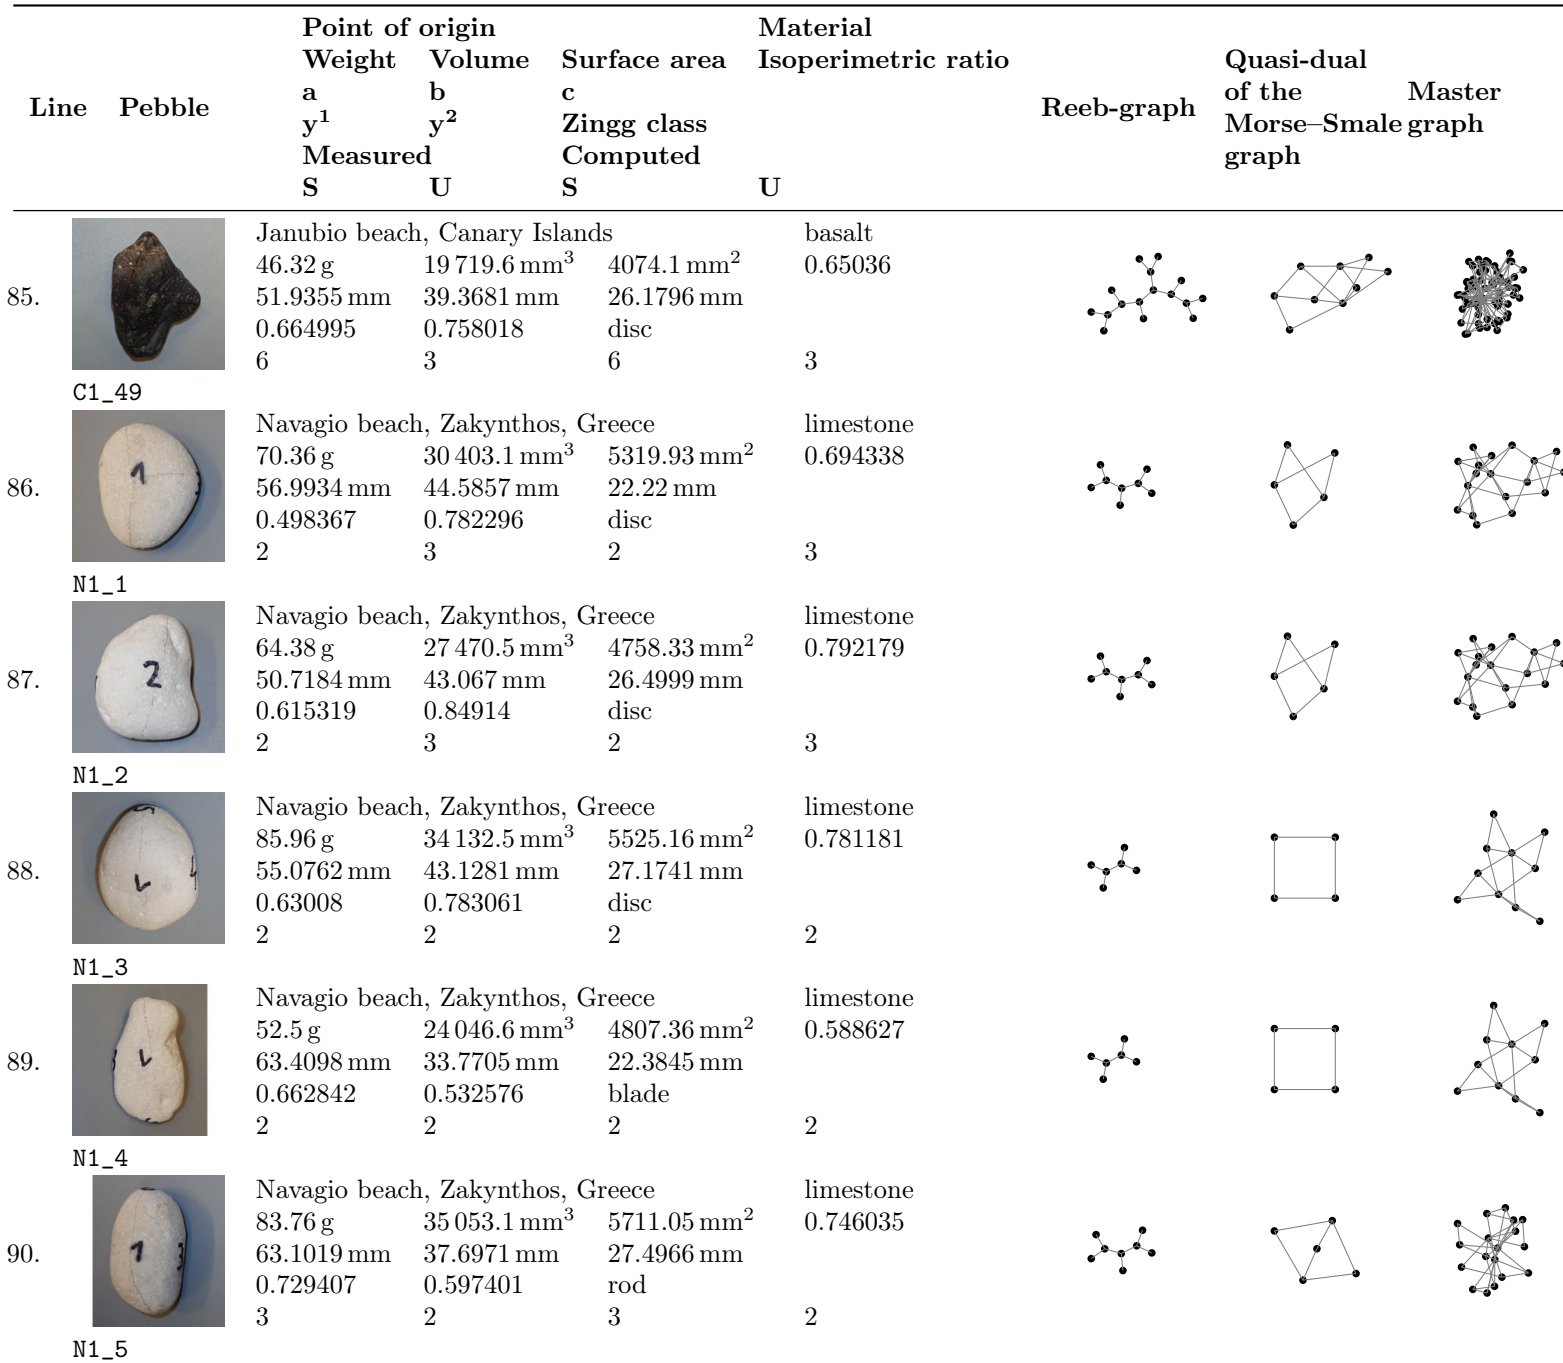   | 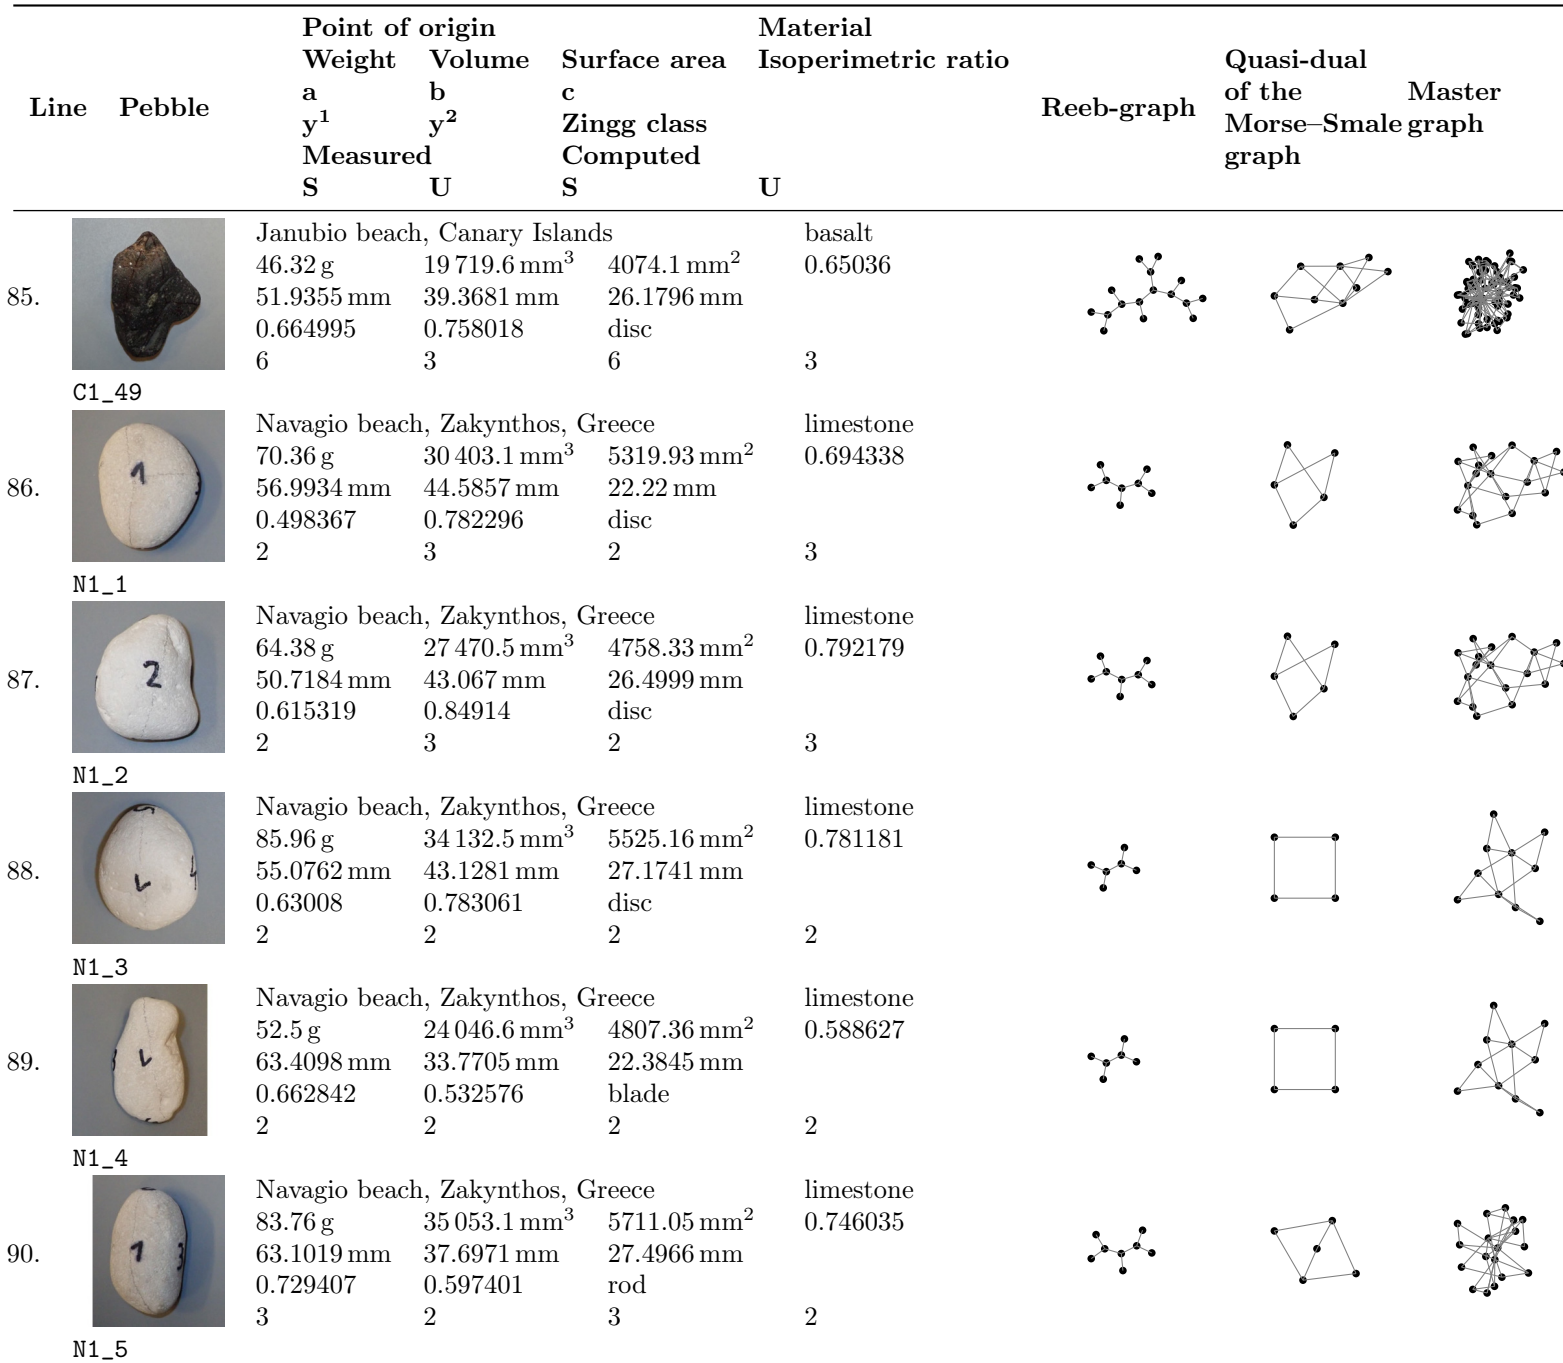   |                 |
|      |                                                                                     | 64.38 g                          | 27 470.5 mm <sup>3</sup> | 4758.33 mm <sup>2</sup> | 0.792179  |                                                                                       |                                                                                       |                                                                                       |                 |
|      |                                                                                     | 50.7184 mm                       | 43.067 mm                | 26.4999 mm              |           |                                                                                       |                                                                                       |                                                                                       |                 |
|      |                                                                                     | 0.615319                         | 0.84914                  | disc                    |           |                                                                                       |                                                                                       |                                                                                       |                 |
|      |                                                                                     | 2                                | 3                        | 2                       | 3         |                                                                                       |                                                                                       |                                                                                       |                 |
| 88.  | 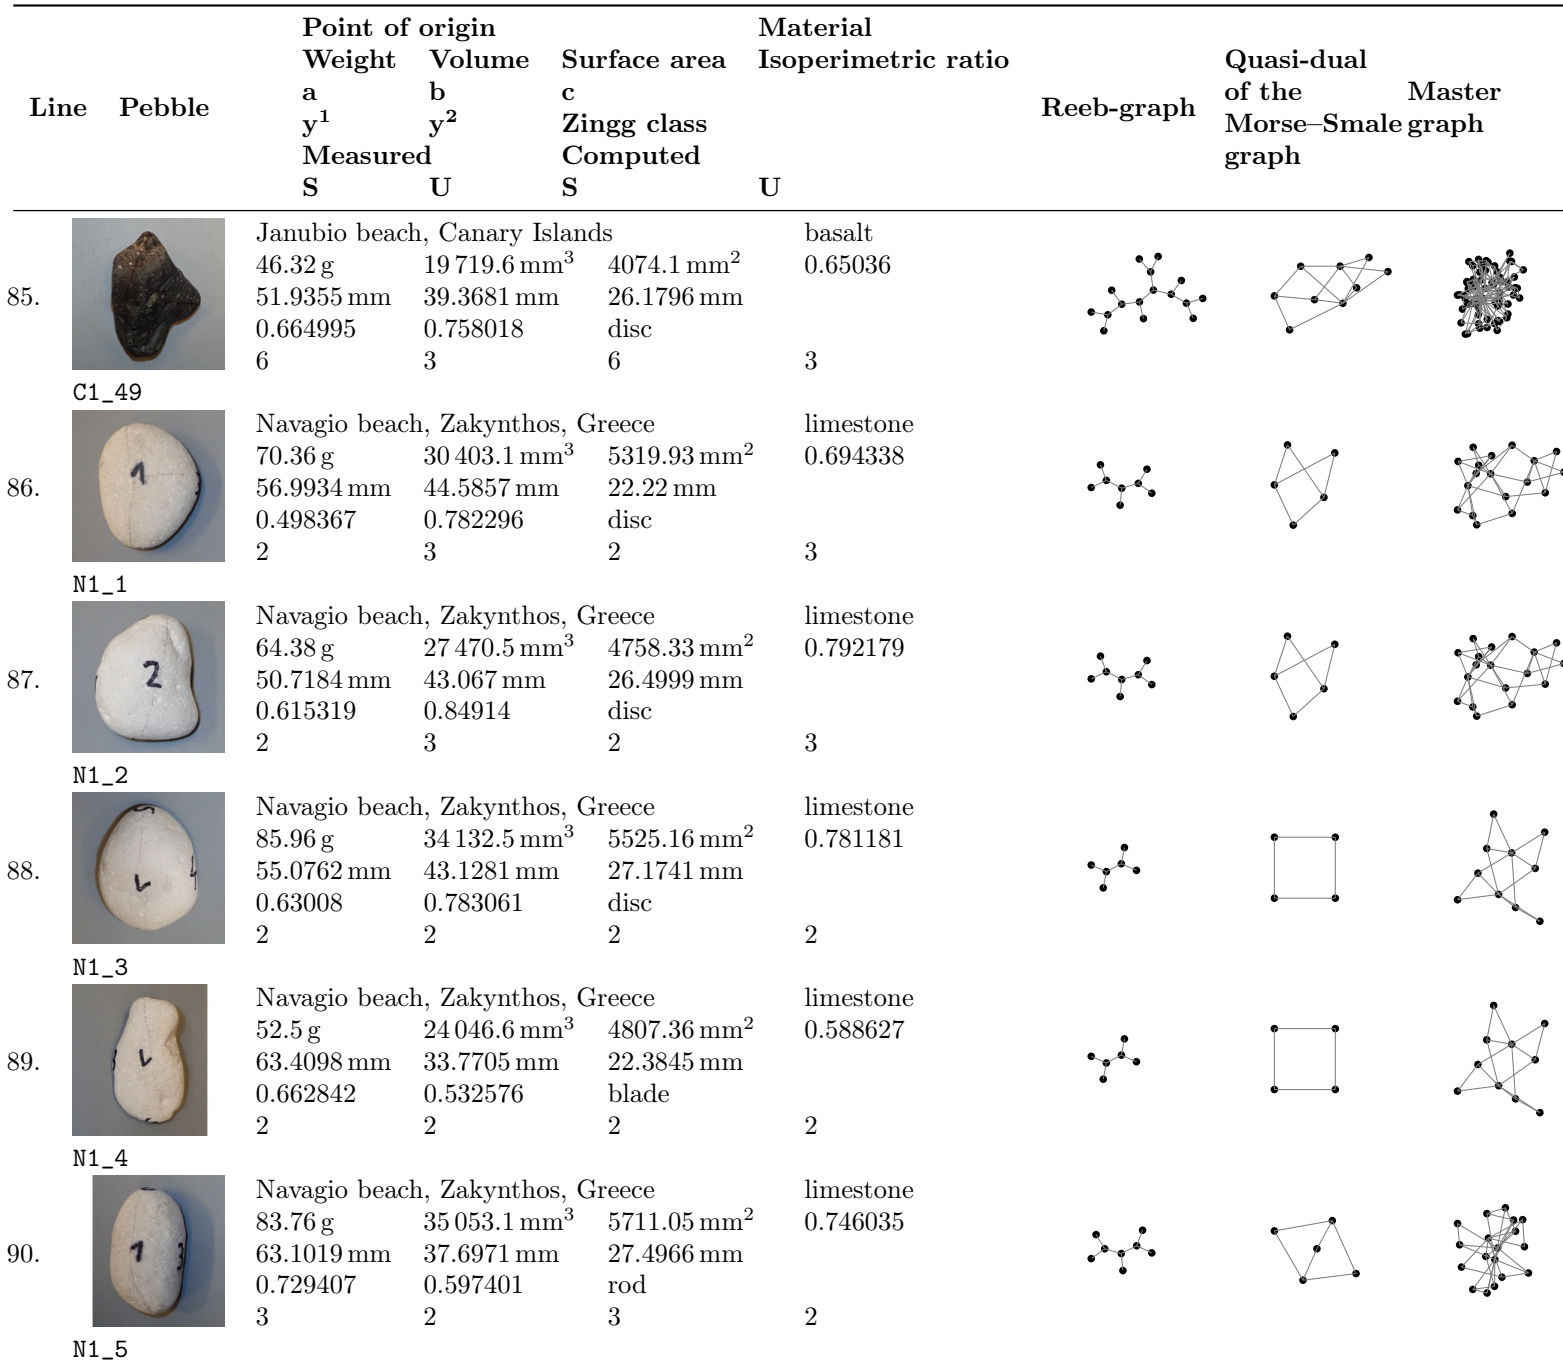  | Navagio beach, Zakynthos, Greece |                          |                         | limestone | 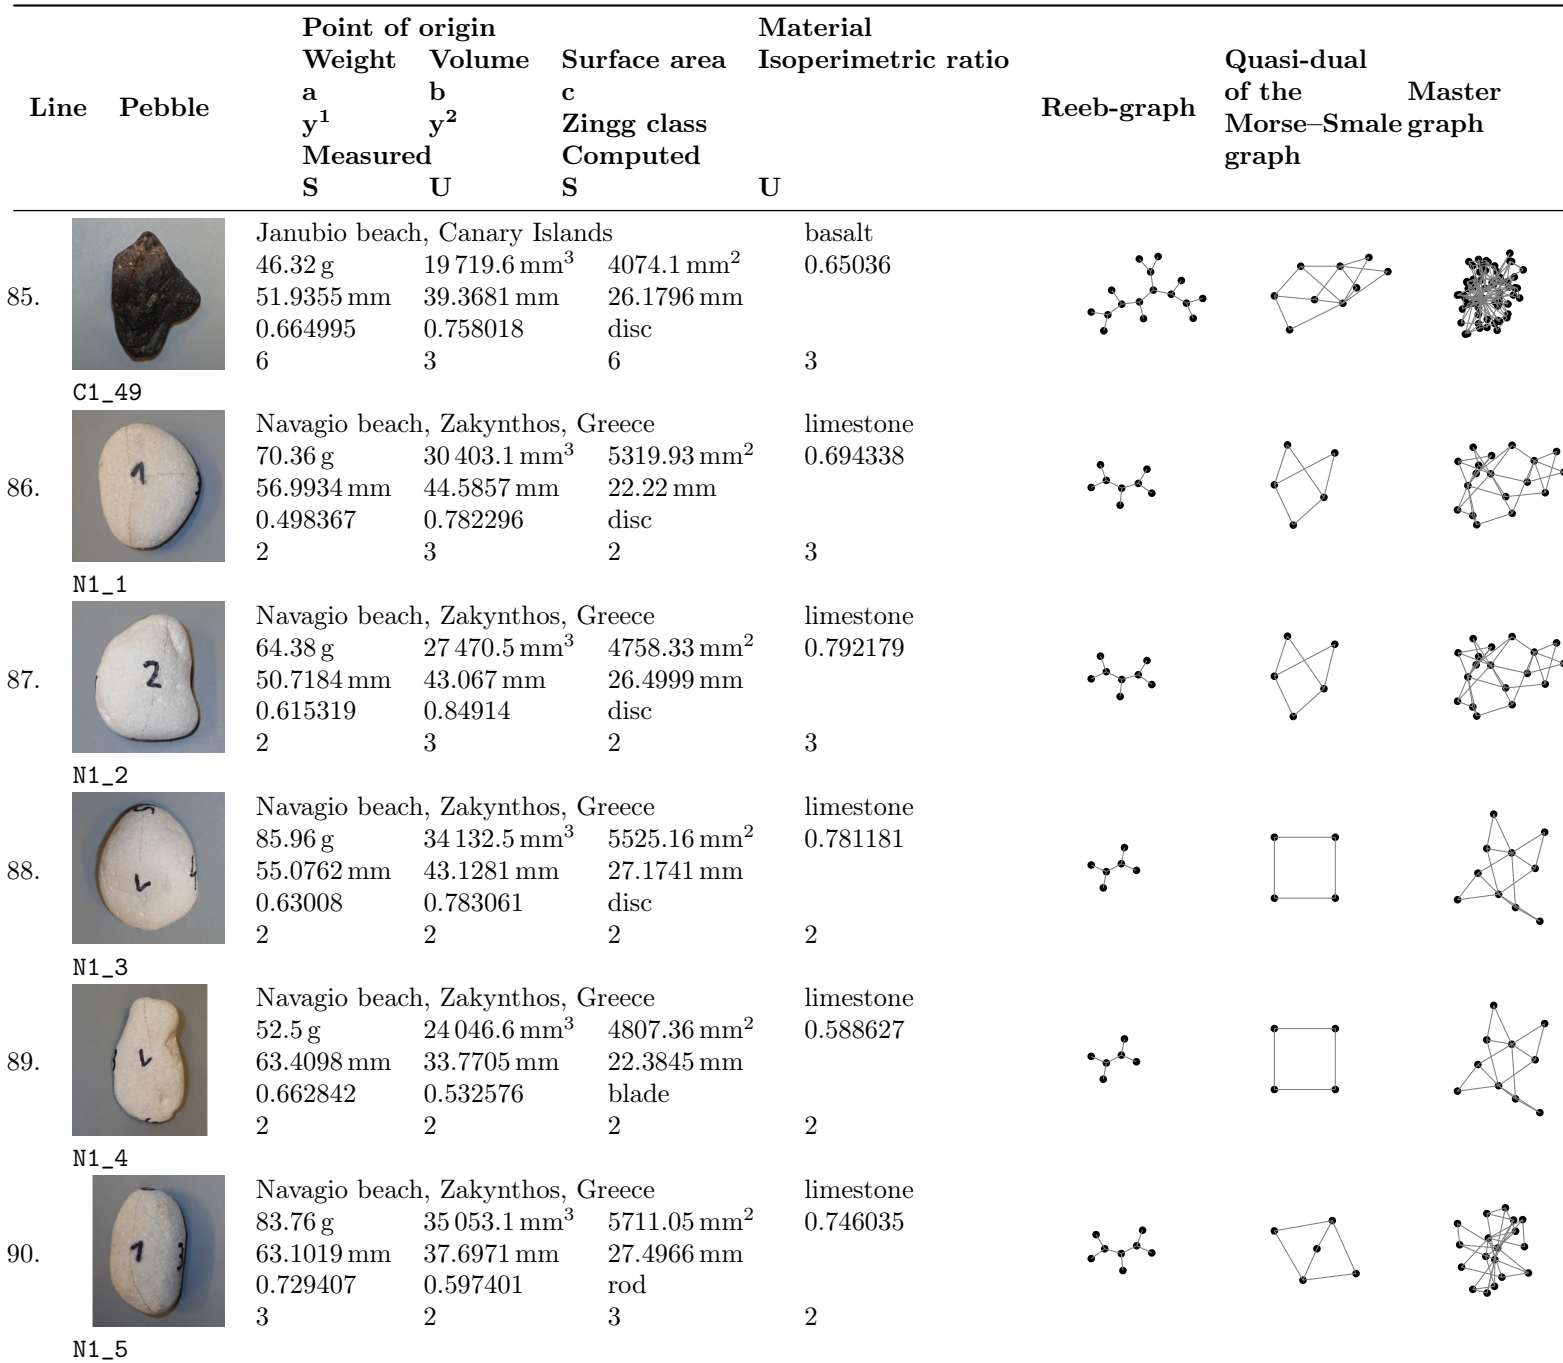  | 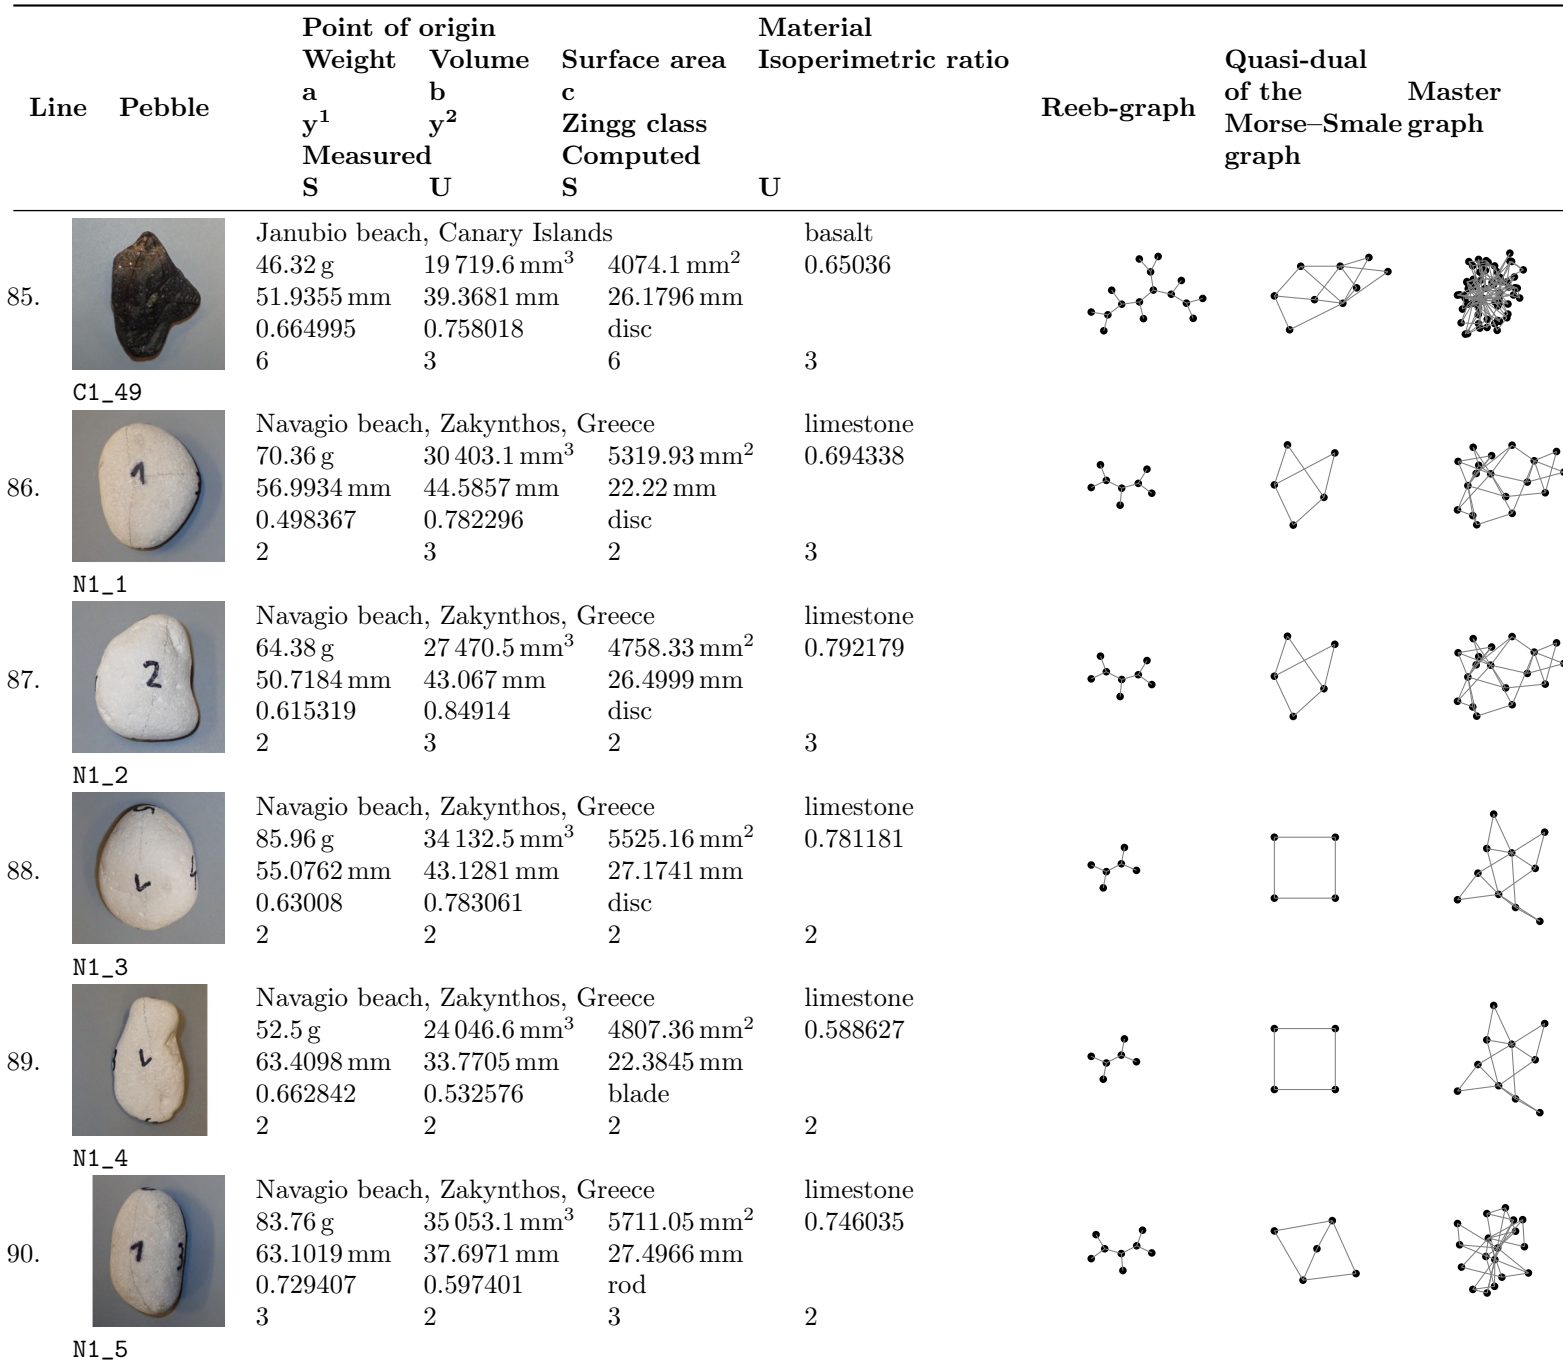  | 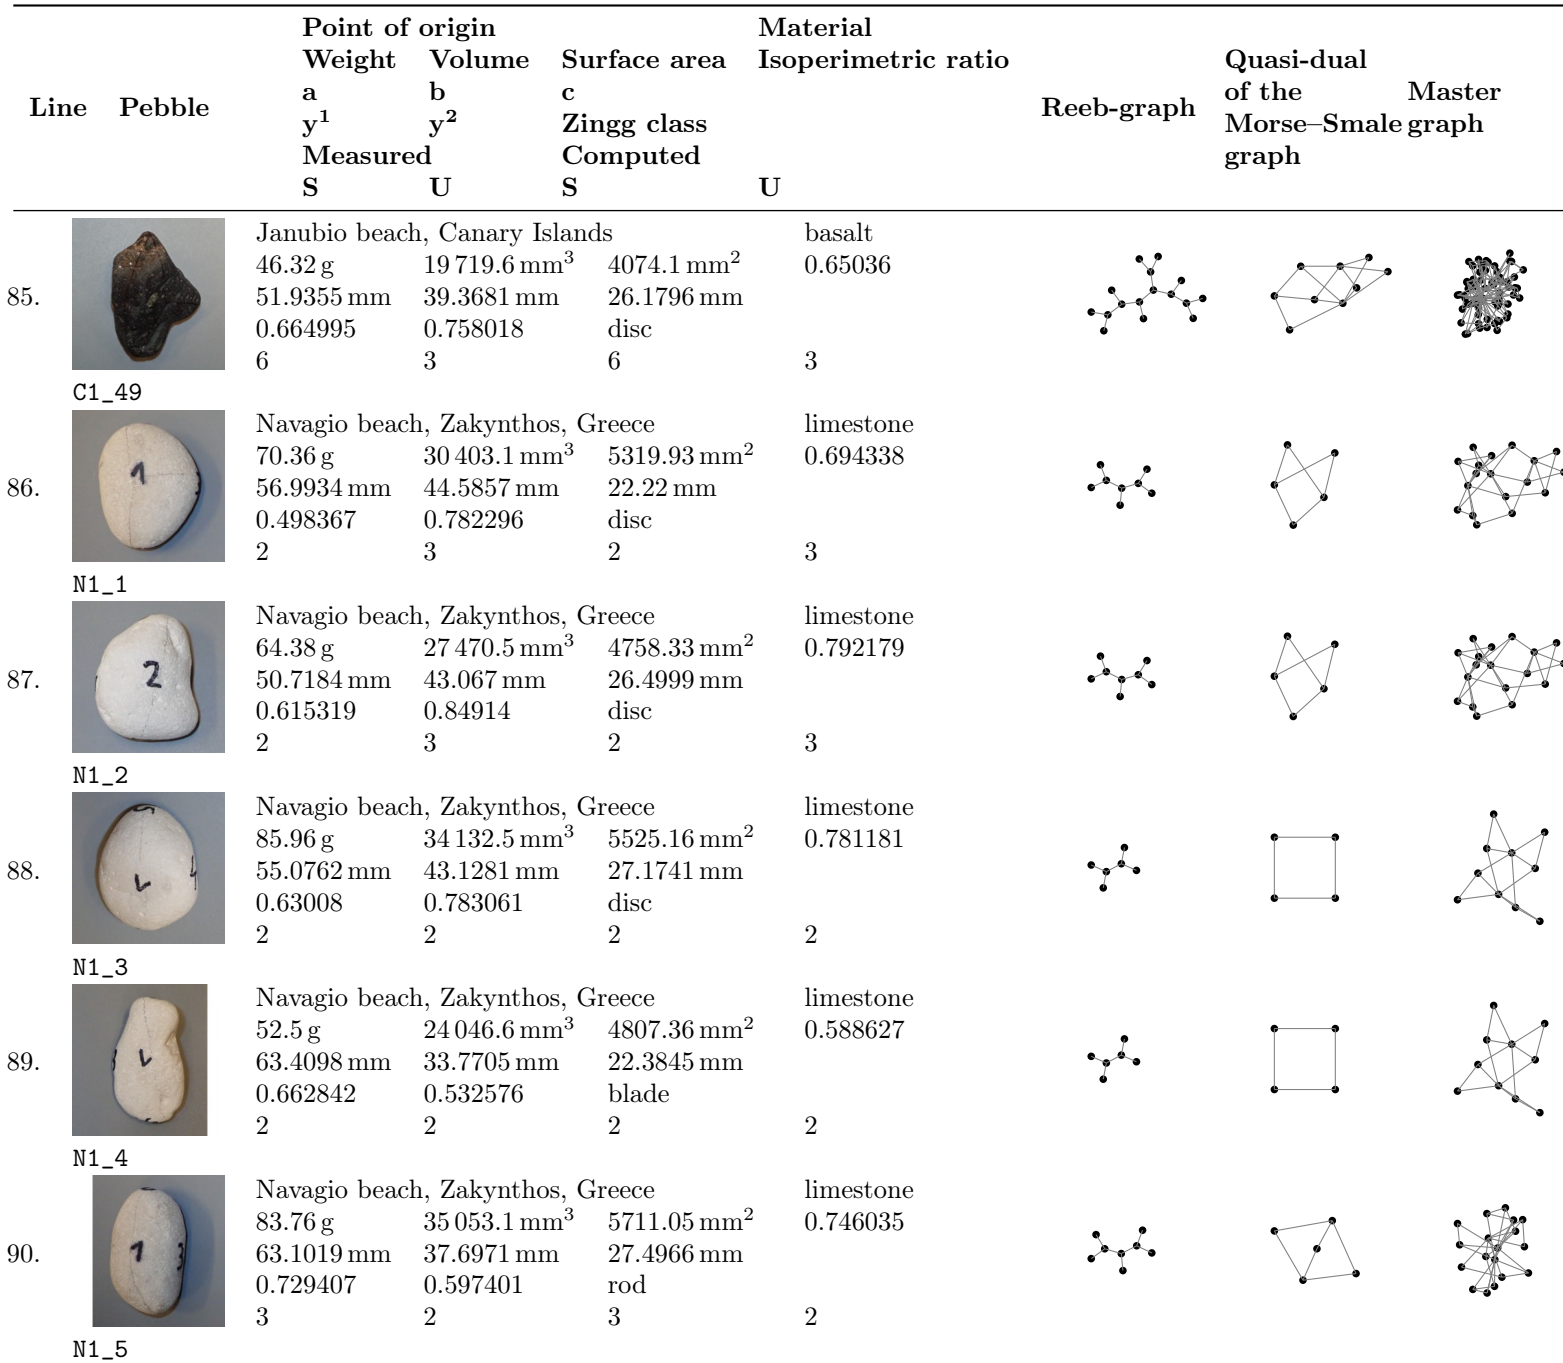  |                 |
|      |                                                                                     | 85.96 g                          | 34 132.5 mm <sup>3</sup> | 5525.16 mm <sup>2</sup> | 0.781181  |                                                                                       |                                                                                       |                                                                                       |                 |
|      |                                                                                     | 55.0762 mm                       | 43.1281 mm               | 27.1741 mm              |           |                                                                                       |                                                                                       |                                                                                       |                 |
|      |                                                                                     | 0.63008                          | 0.783061                 | disc                    |           |                                                                                       |                                                                                       |                                                                                       |                 |
|      |                                                                                     | 2                                | 2                        | 2                       | 2         |                                                                                       |                                                                                       |                                                                                       |                 |
| 89.  | 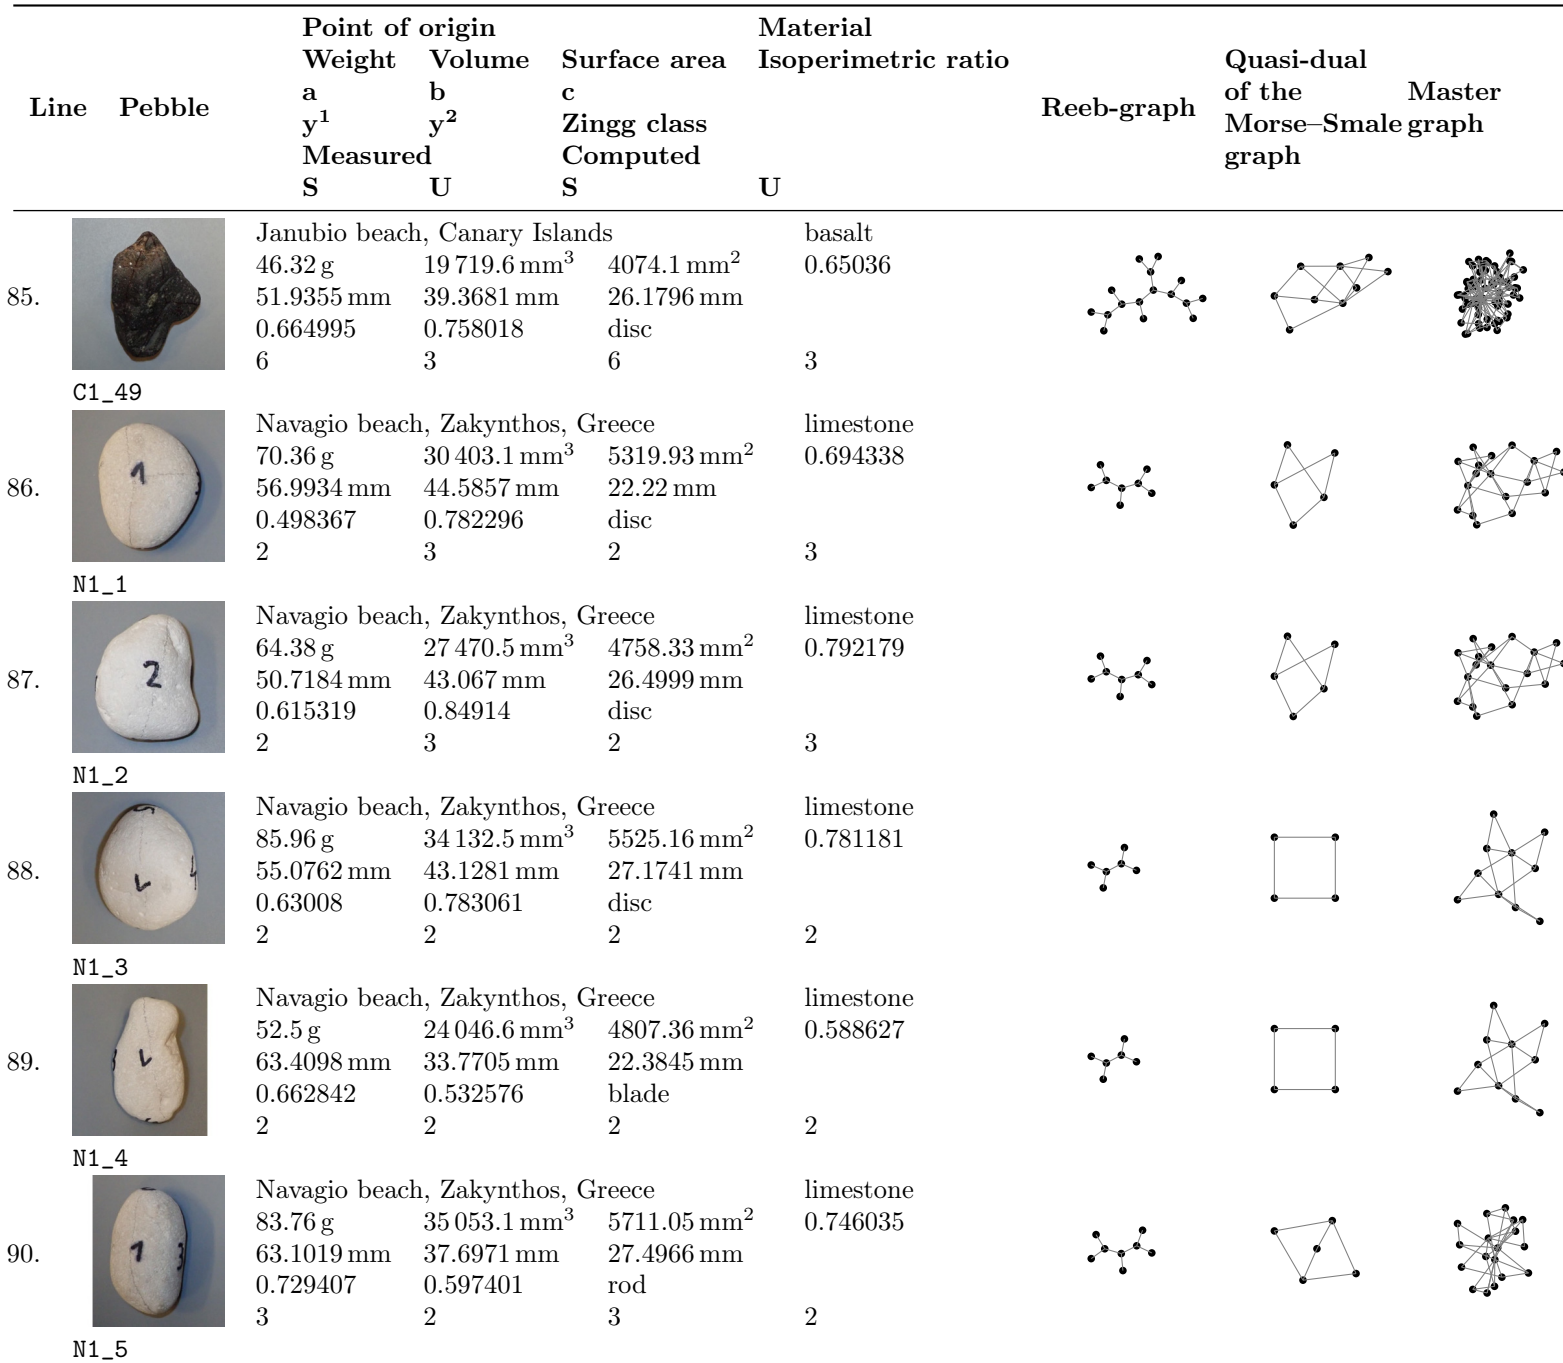 | Navagio beach, Zakynthos, Greece |                          |                         | limestone | 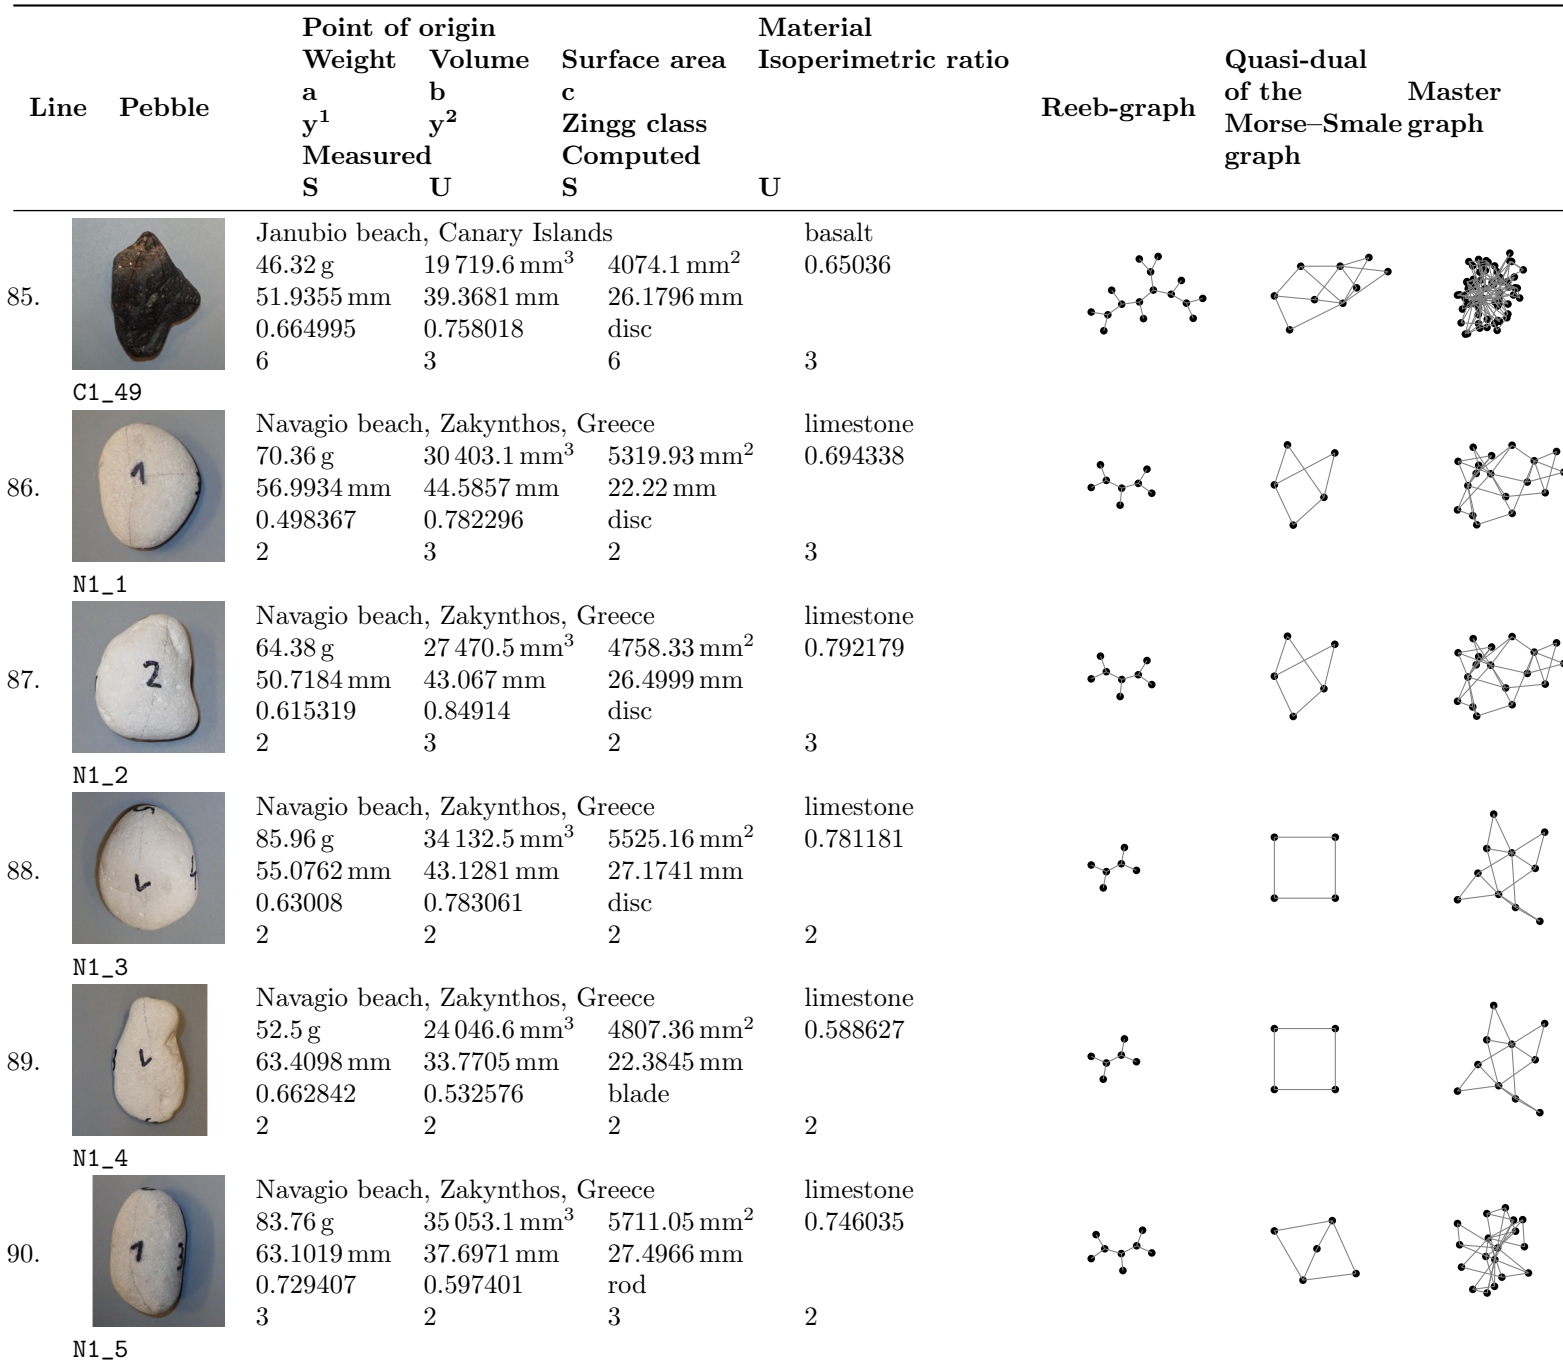 | 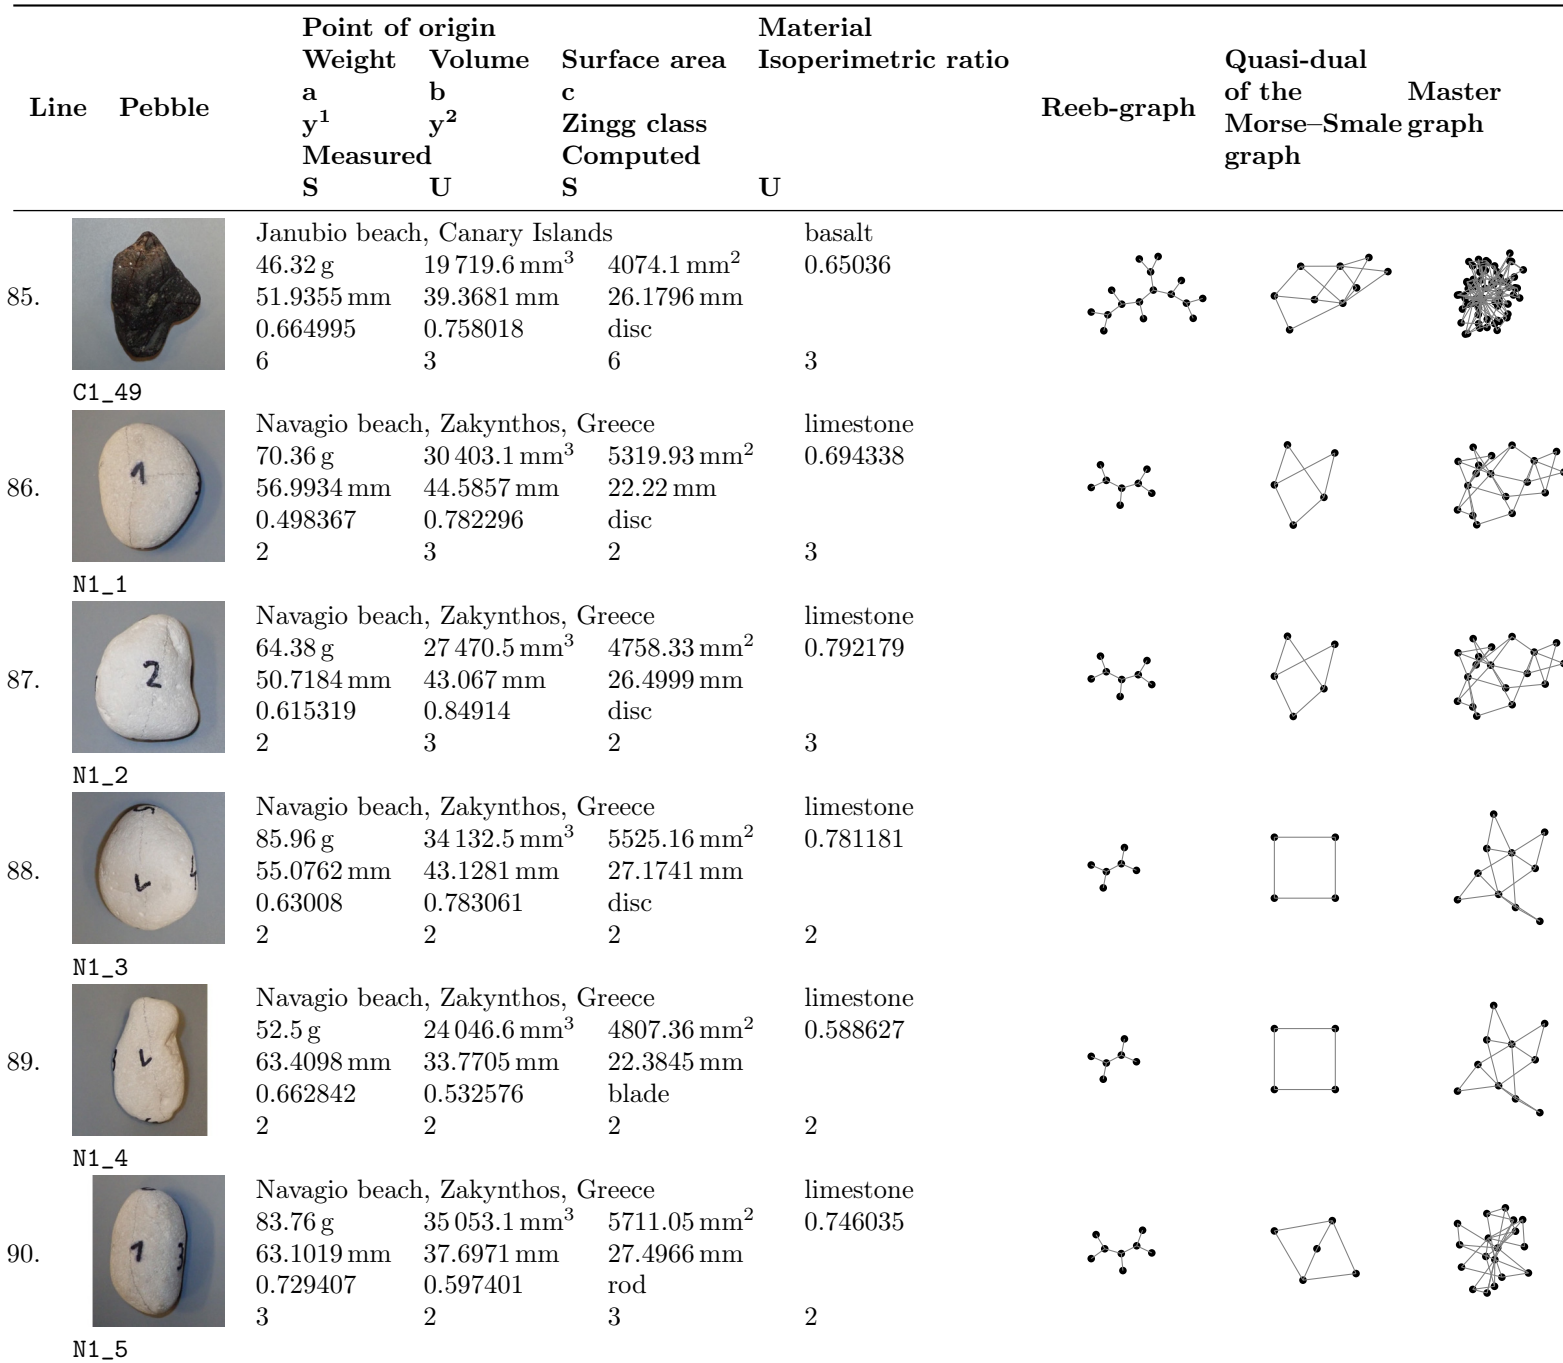 | 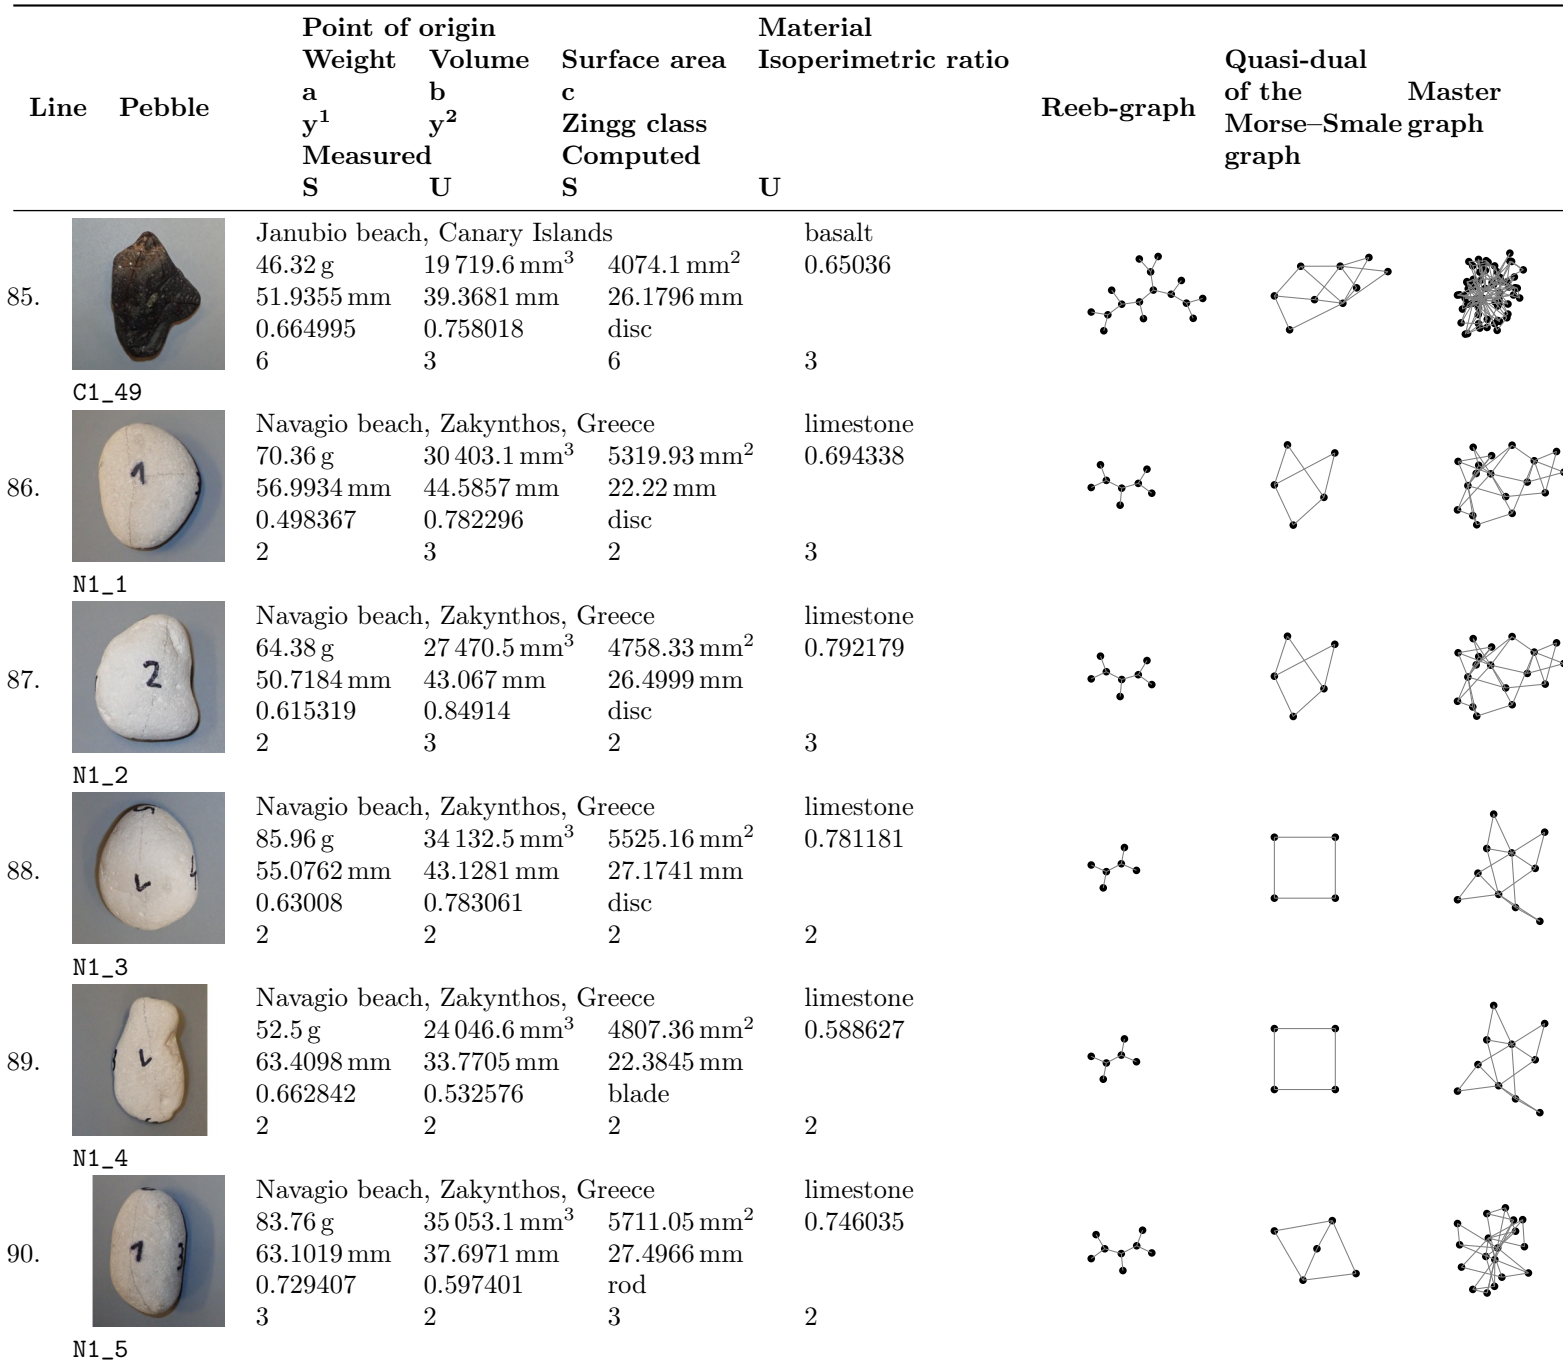 |                 |
|      |                                                                                     | 52.5 g                           | 24 046.6 mm <sup>3</sup> | 4807.36 mm <sup>2</sup> | 0.588627  |                                                                                       |                                                                                       |                                                                                       |                 |
|      |                                                                                     | 63.4098 mm                       | 33.7705 mm               | 22.3845 mm              |           |                                                                                       |                                                                                       |                                                                                       |                 |
|      |                                                                                     | 0.662842                         | 0.532576                 | blade                   |           |                                                                                       |                                                                                       |                                                                                       |                 |
|      |                                                                                     | 2                                | 2                        | 2                       | 2         |                                                                                       |                                                                                       |                                                                                       |                 |
| 90.  | 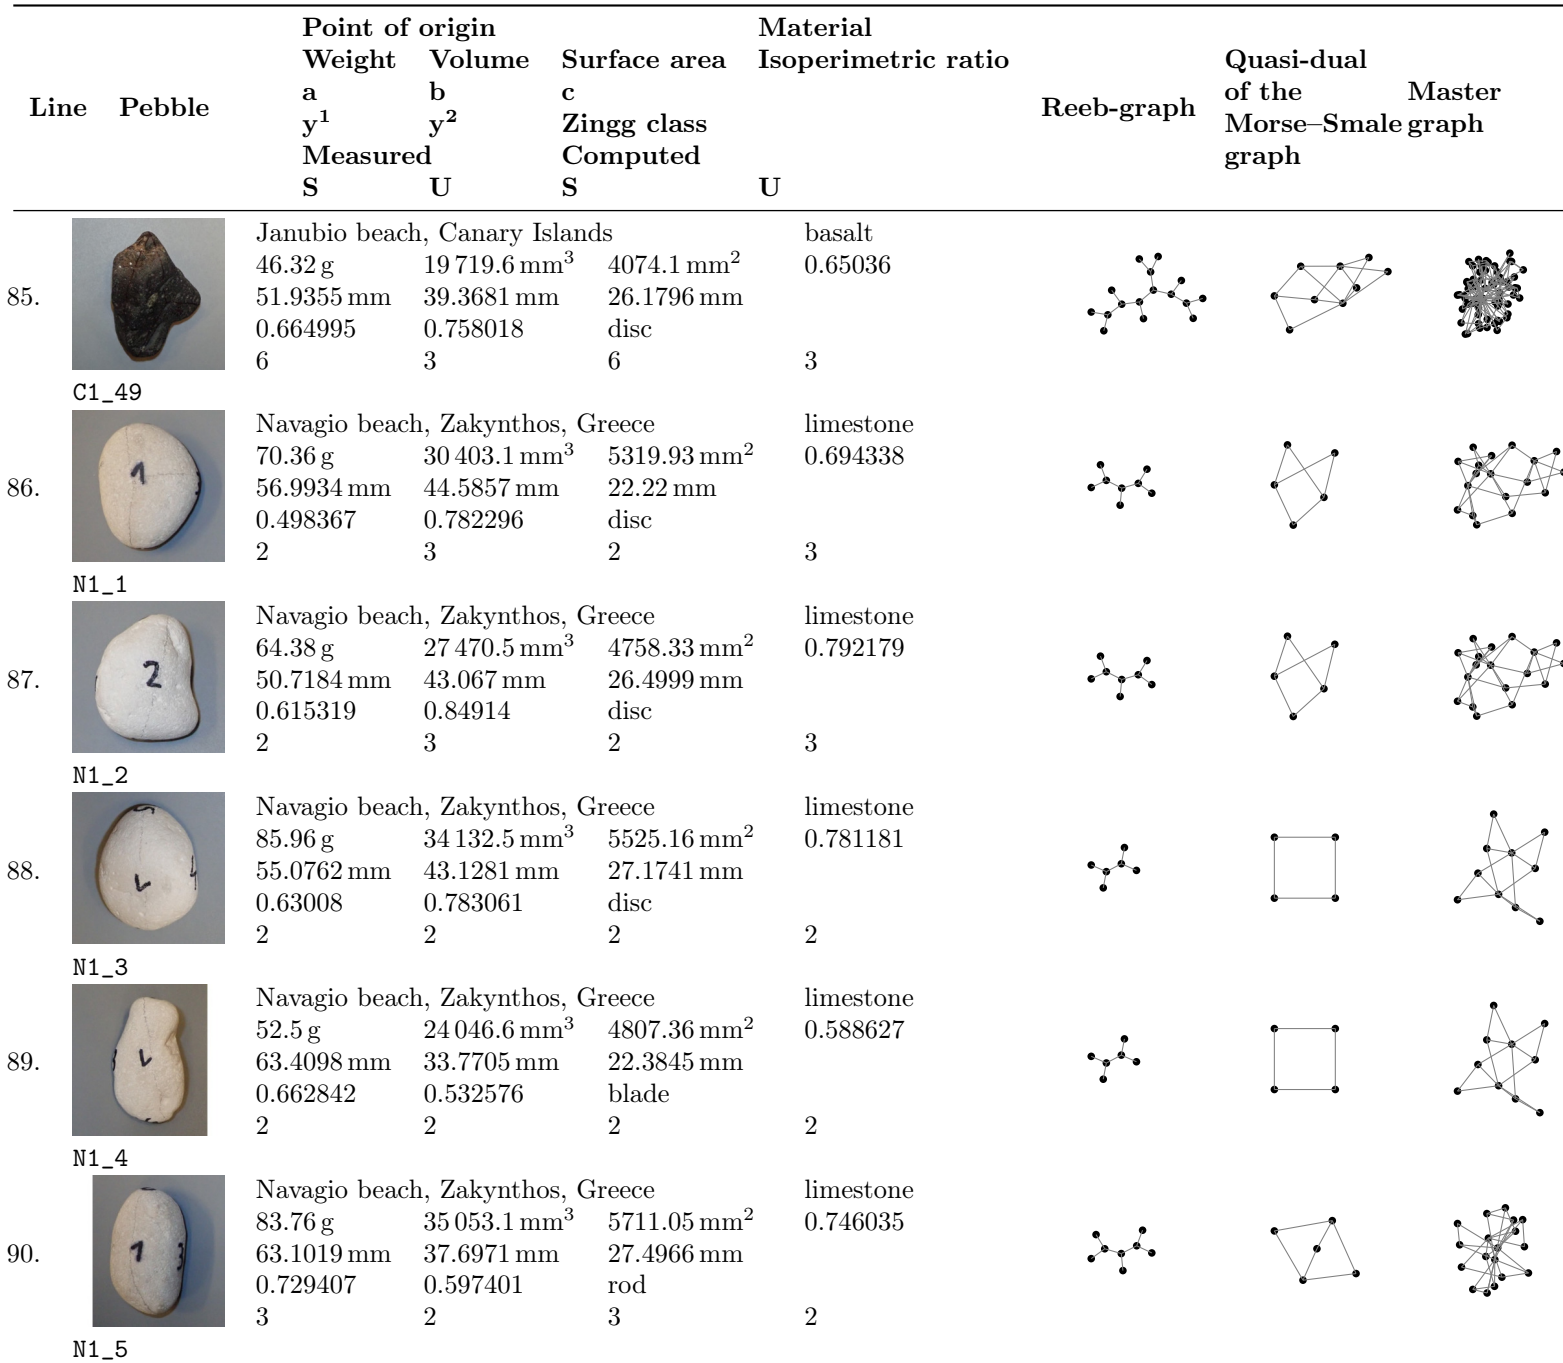 | Navagio beach, Zakynthos, Greece |                          |                         | limestone | 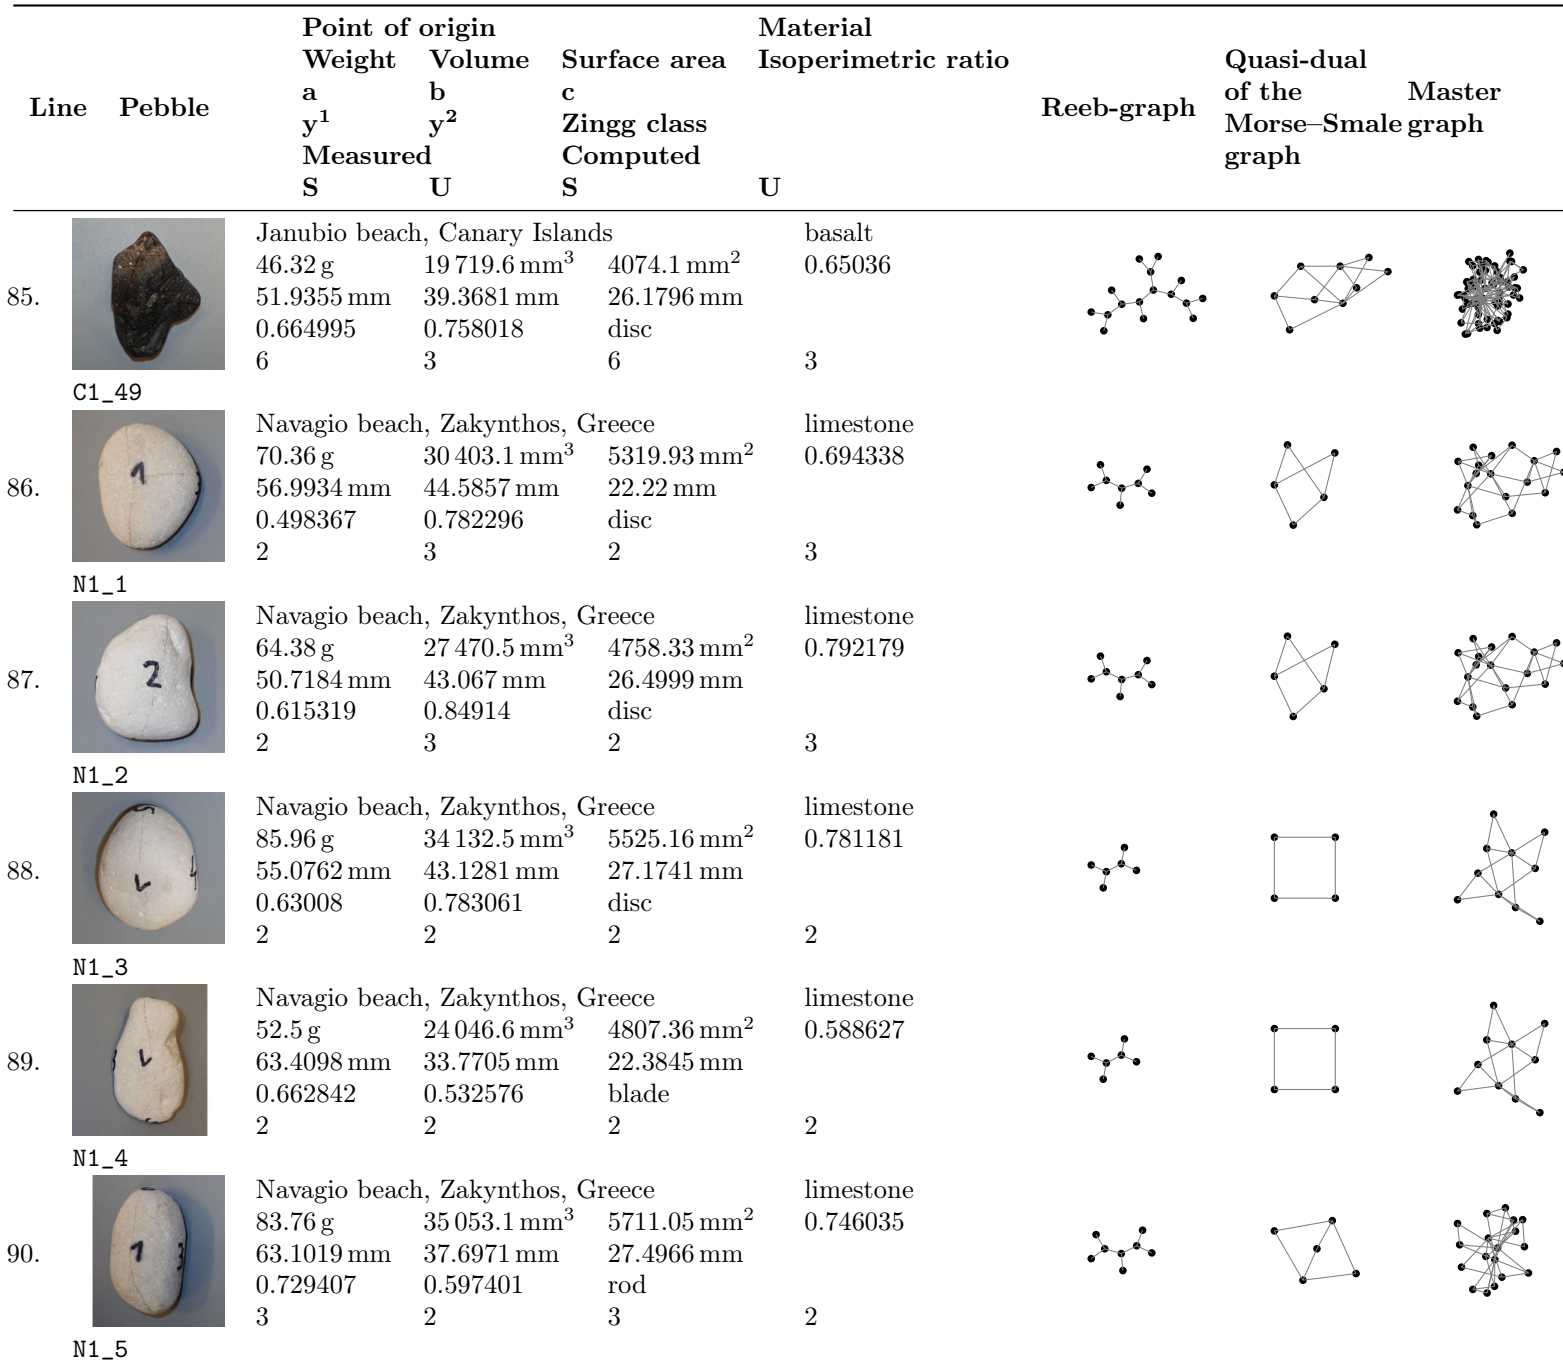 | 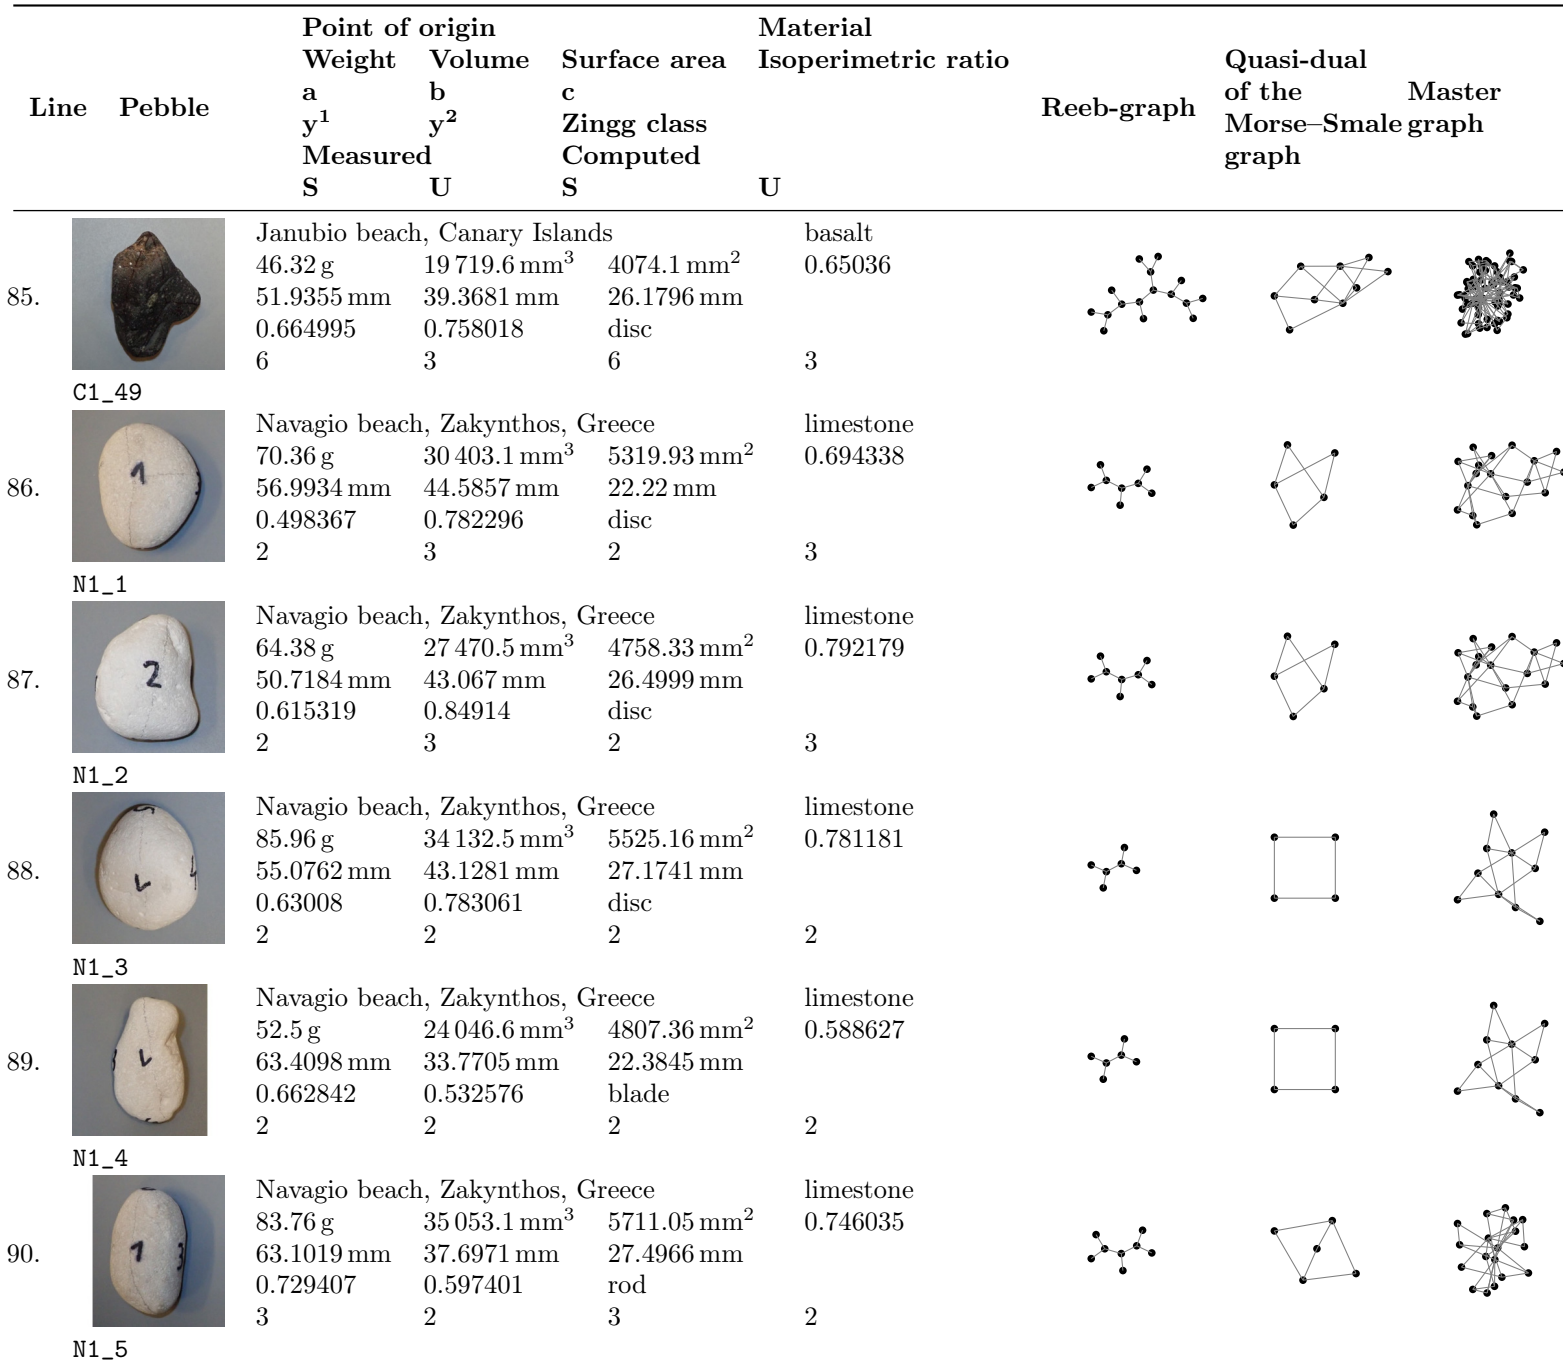 | 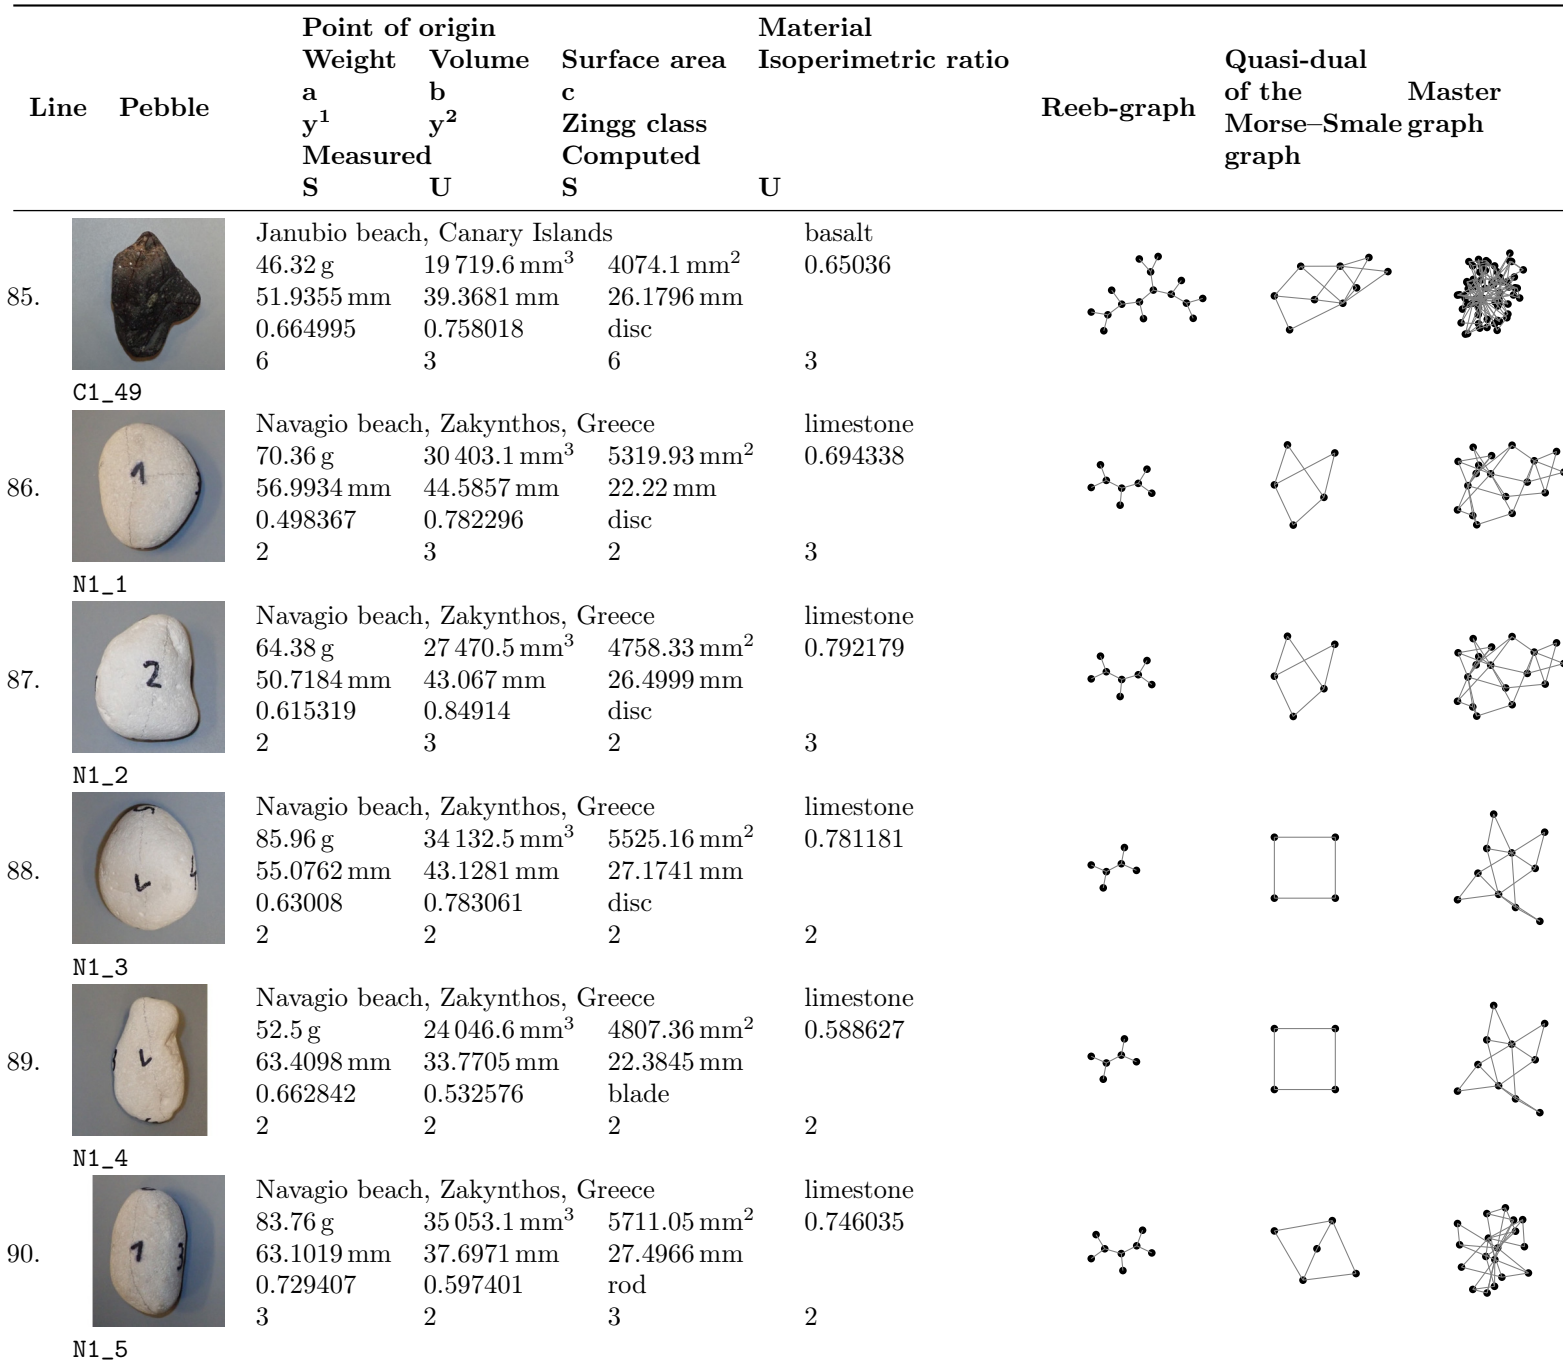 |                 |
|      |                                                                                     | 83.76 g                          | 35 053.1 mm <sup>3</sup> | 5711.05 mm <sup>2</sup> | 0.746035  |                                                                                       |                                                                                       |                                                                                       |                 |
|      |                                                                                     | 63.1019 mm                       | 37.6971 mm               | 27.4966 mm              |           |                                                                                       |                                                                                       |                                                                                       |                 |
|      |                                                                                     | 0.729407                         | 0.597401                 | rod                     |           |                                                                                       |                                                                                       |                                                                                       |                 |
|      |                                                                                     | 3                                | 2                        | 3                       | 2         |                                                                                       |                                                                                       |                                                                                       |                 |
|      | N1_5                                                                                |                                  |                          |                         |           |                                                                                       |                                                                                       |                                                                                       |                 |

| Line | Pebble                                                                              | Point of origin                      |                          | Surface area<br>c<br>Zingg class<br>Computed<br>S | Material<br>Isoperimetric ratio<br>U | Reeb-graph                                                                            | Quasi-dual<br>of the<br>Morse–Smale<br>graph                                          | Master<br>graph                                                                       |
|------|-------------------------------------------------------------------------------------|--------------------------------------|--------------------------|---------------------------------------------------|--------------------------------------|---------------------------------------------------------------------------------------|---------------------------------------------------------------------------------------|---------------------------------------------------------------------------------------|
|      |                                                                                     | Weight                               | Volume                   |                                                   |                                      |                                                                                       |                                                                                       |                                                                                       |
|      |                                                                                     | a<br>y <sup>1</sup><br>Measured<br>S | b<br>y <sup>2</sup><br>U |                                                   |                                      |                                                                                       |                                                                                       |                                                                                       |
|      |                                                                                     |                                      |                          |                                                   |                                      |                                                                                       |                                                                                       |                                                                                       |
| 91.  | 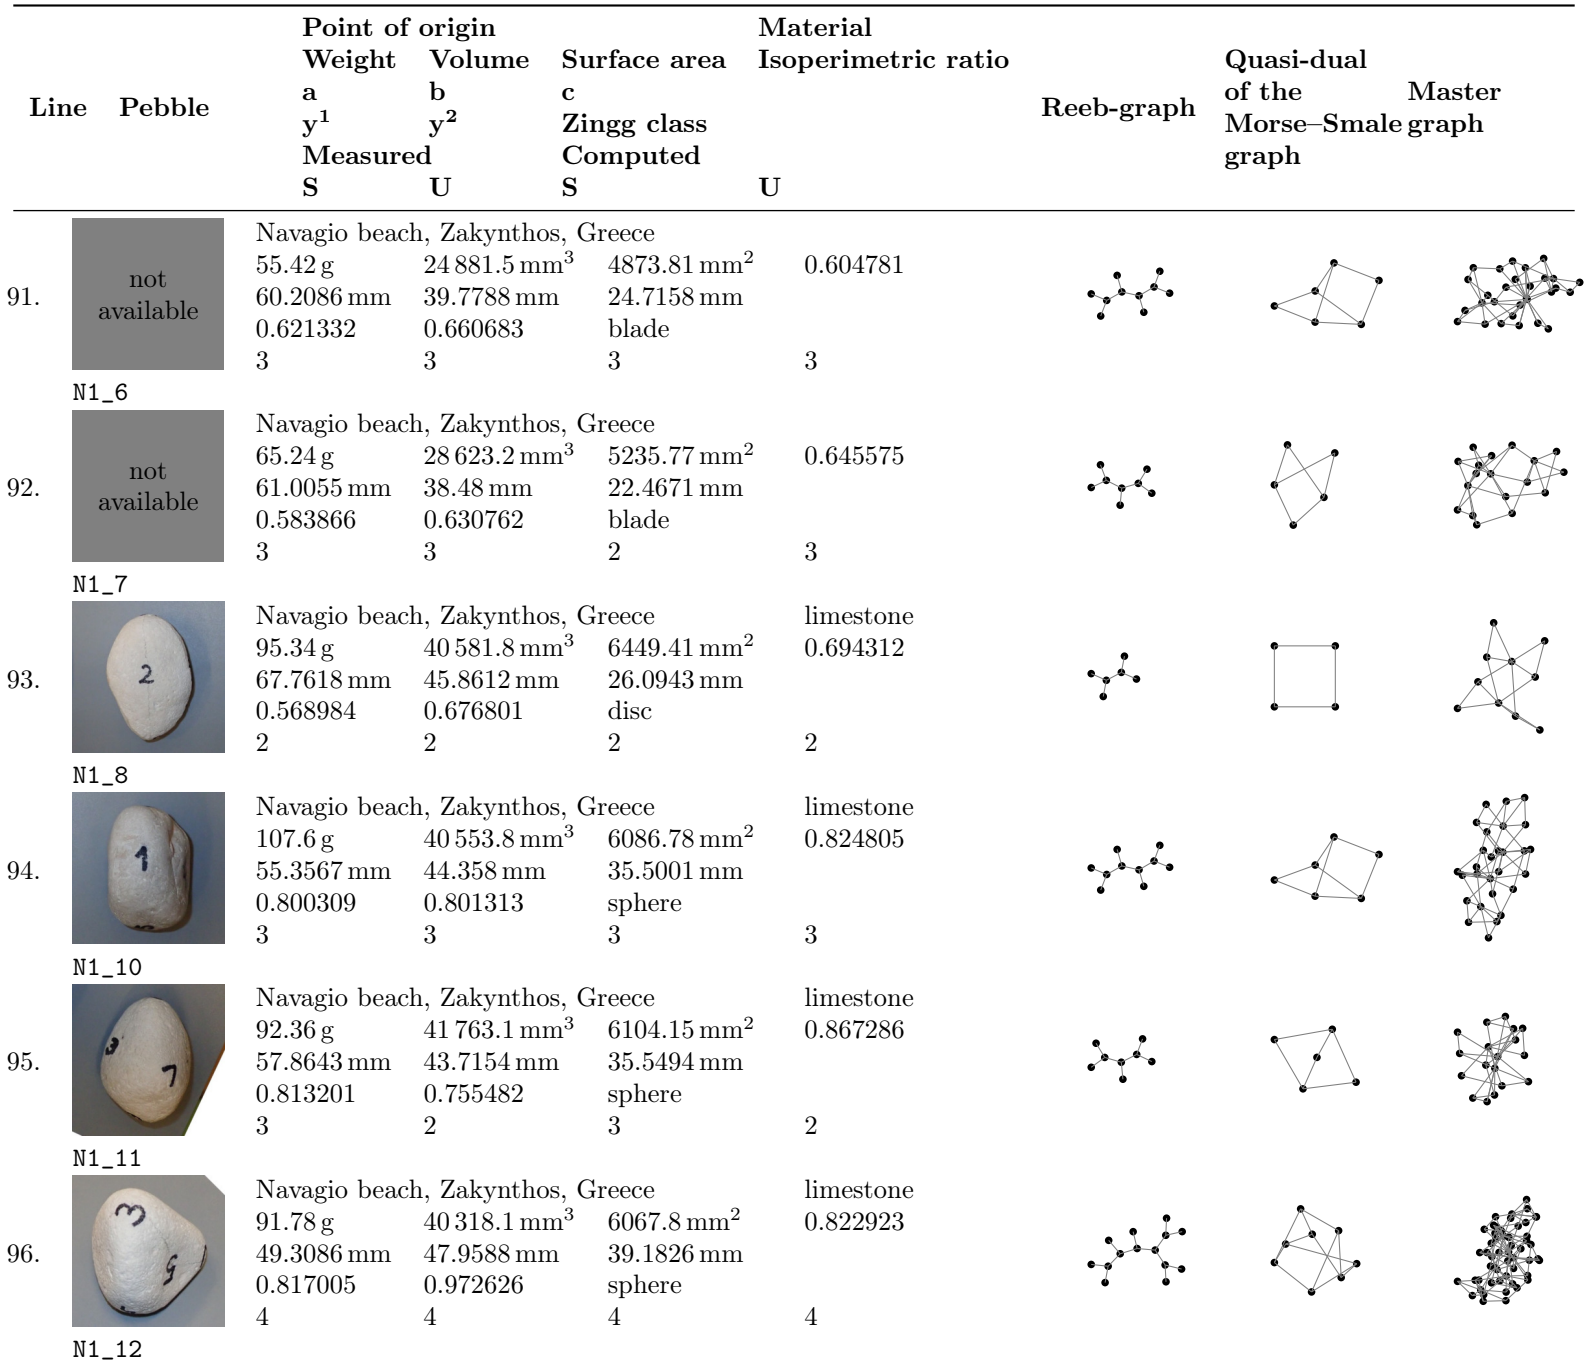   | Navagio beach, Zakynthos, Greece     |                          |                                                   | 0.604781                             | 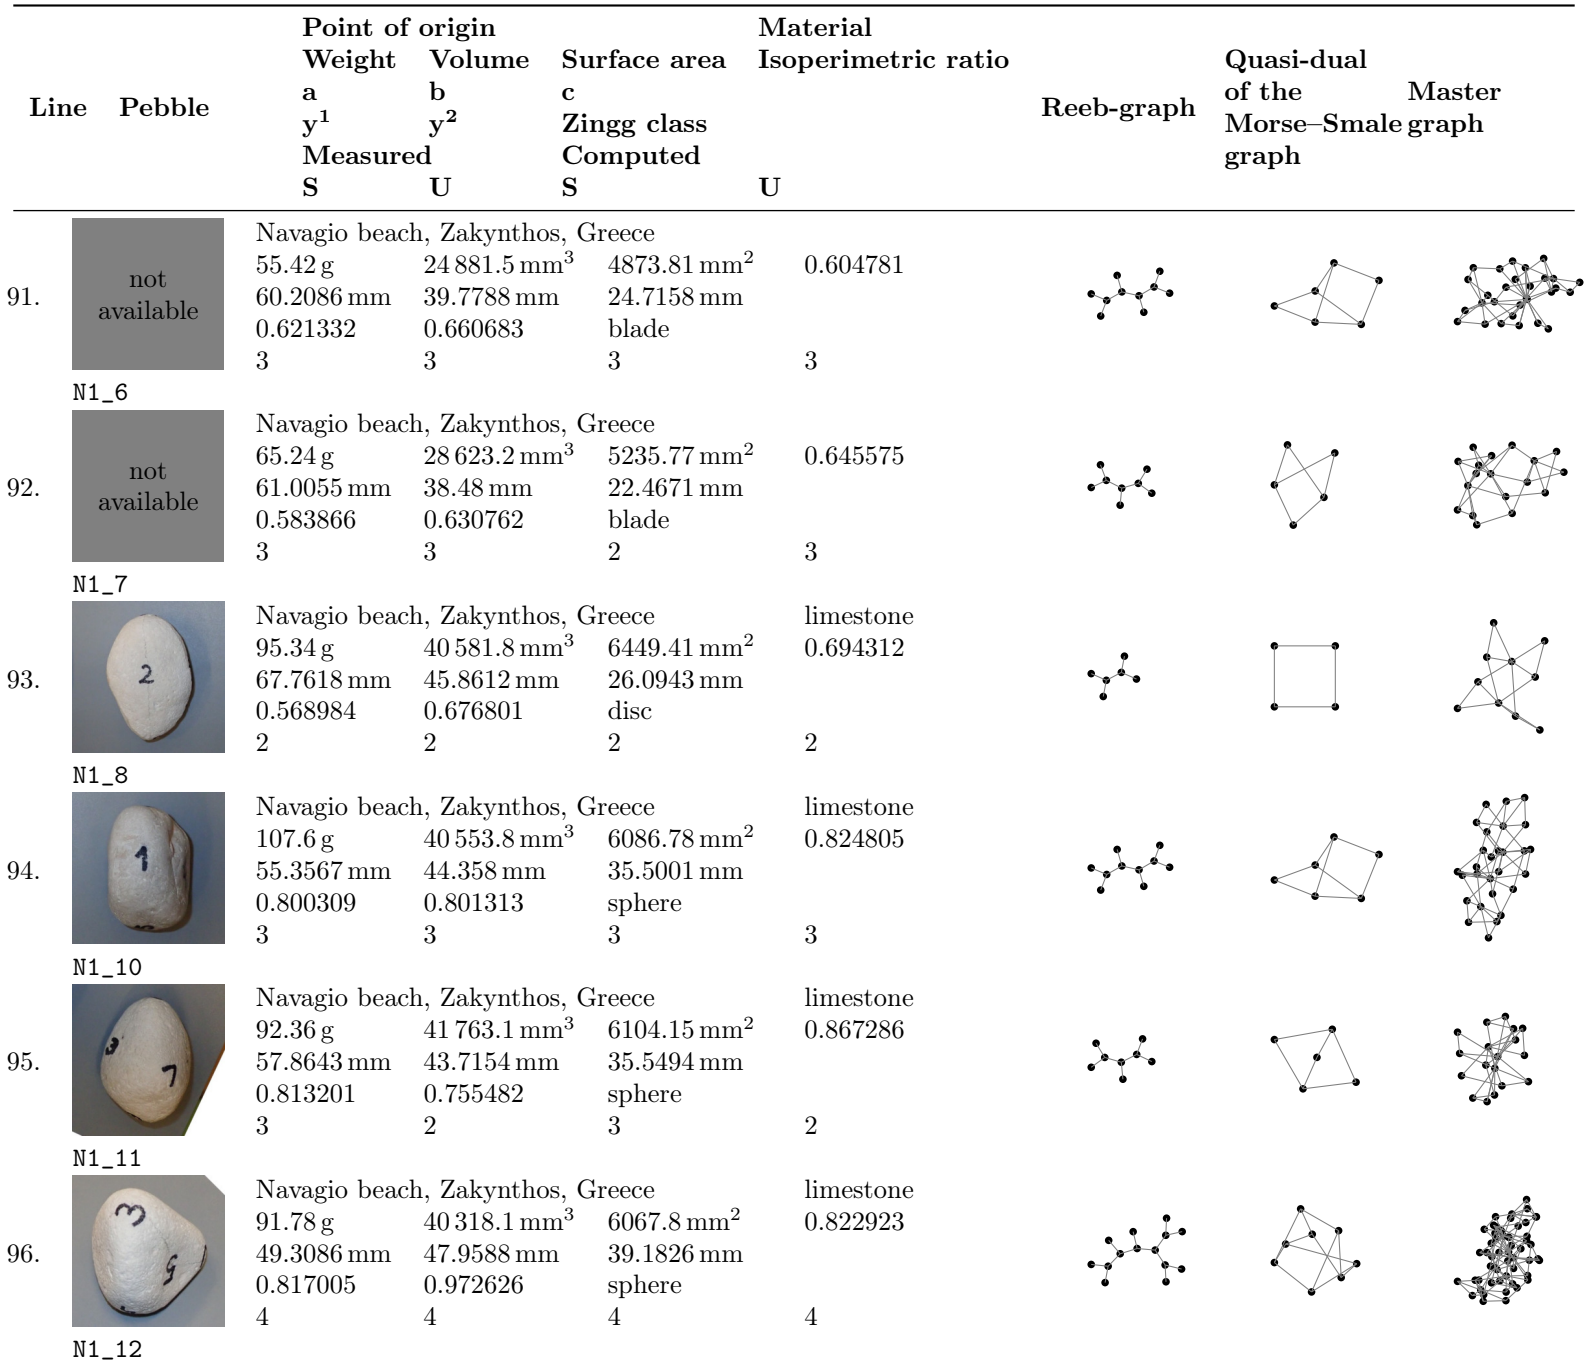   | 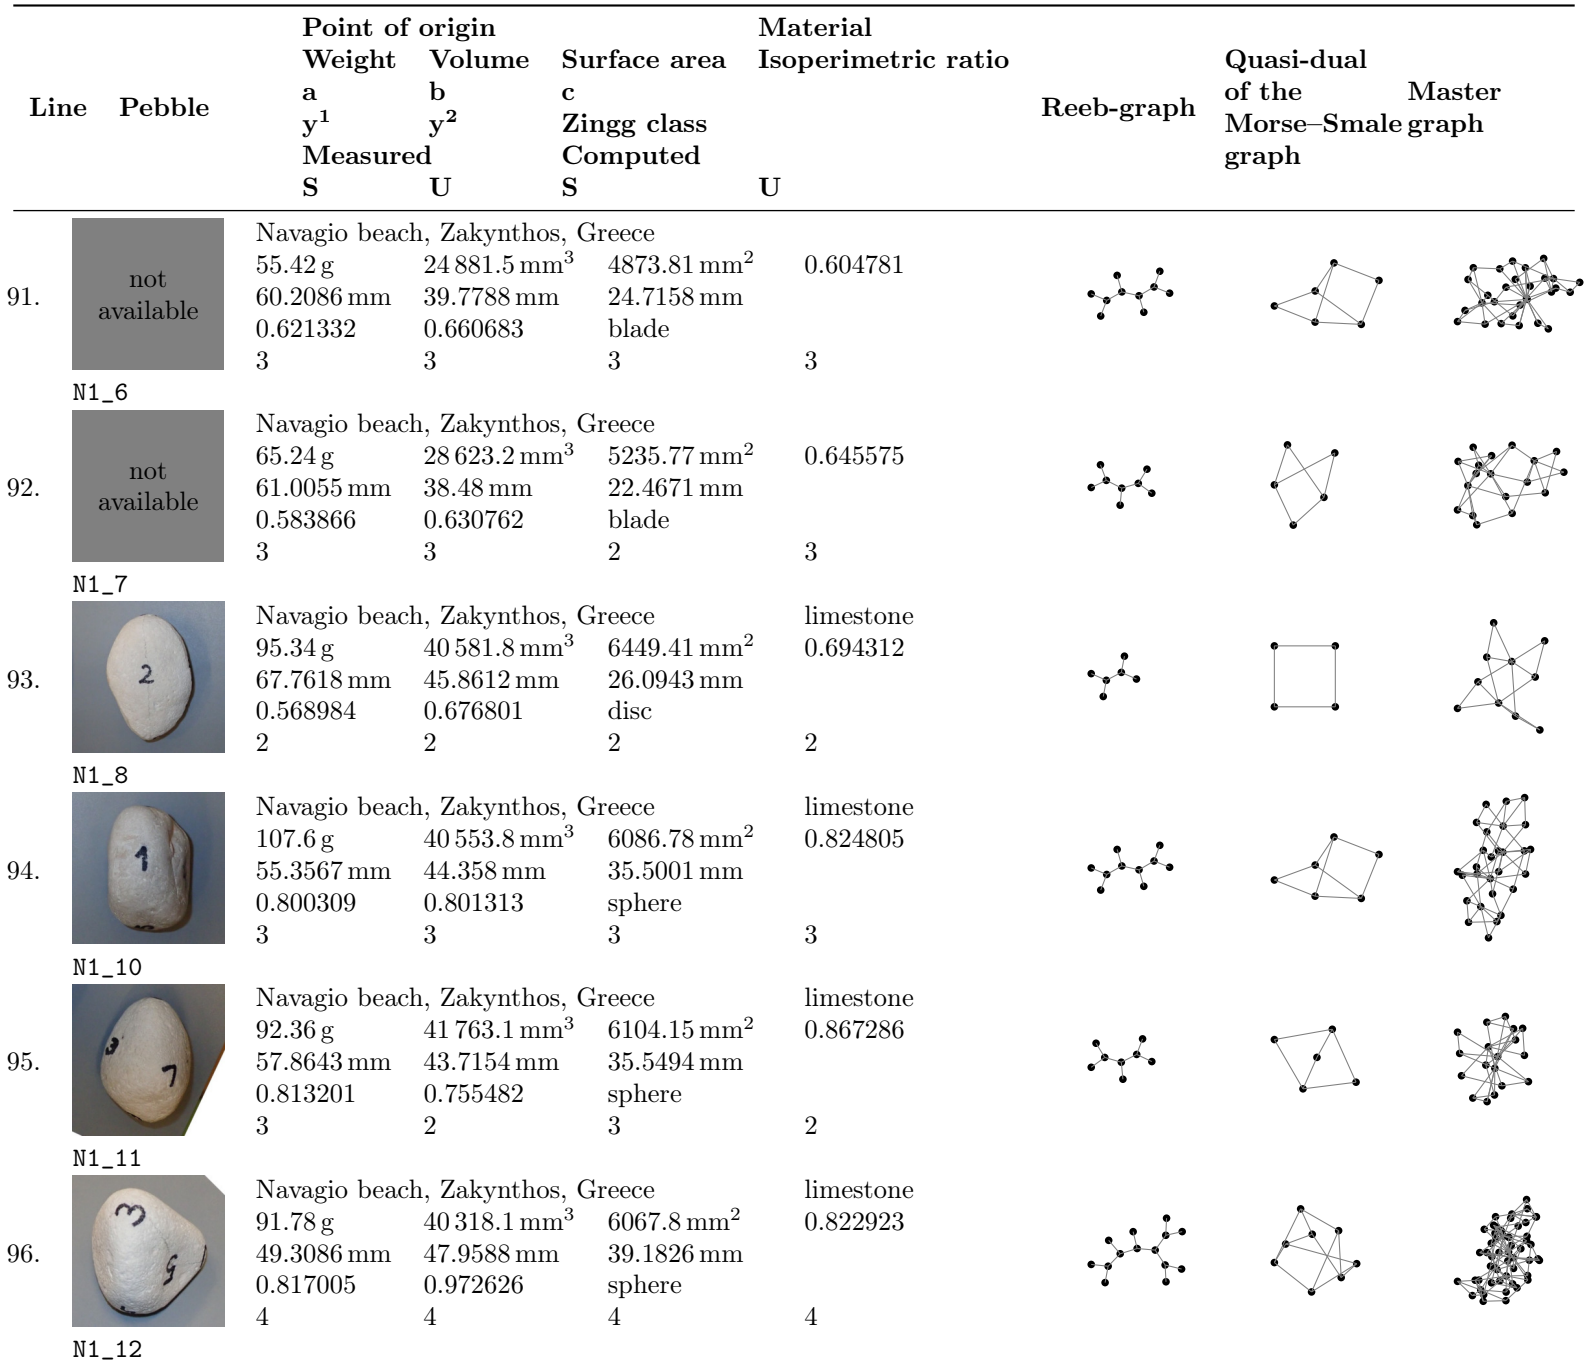   | 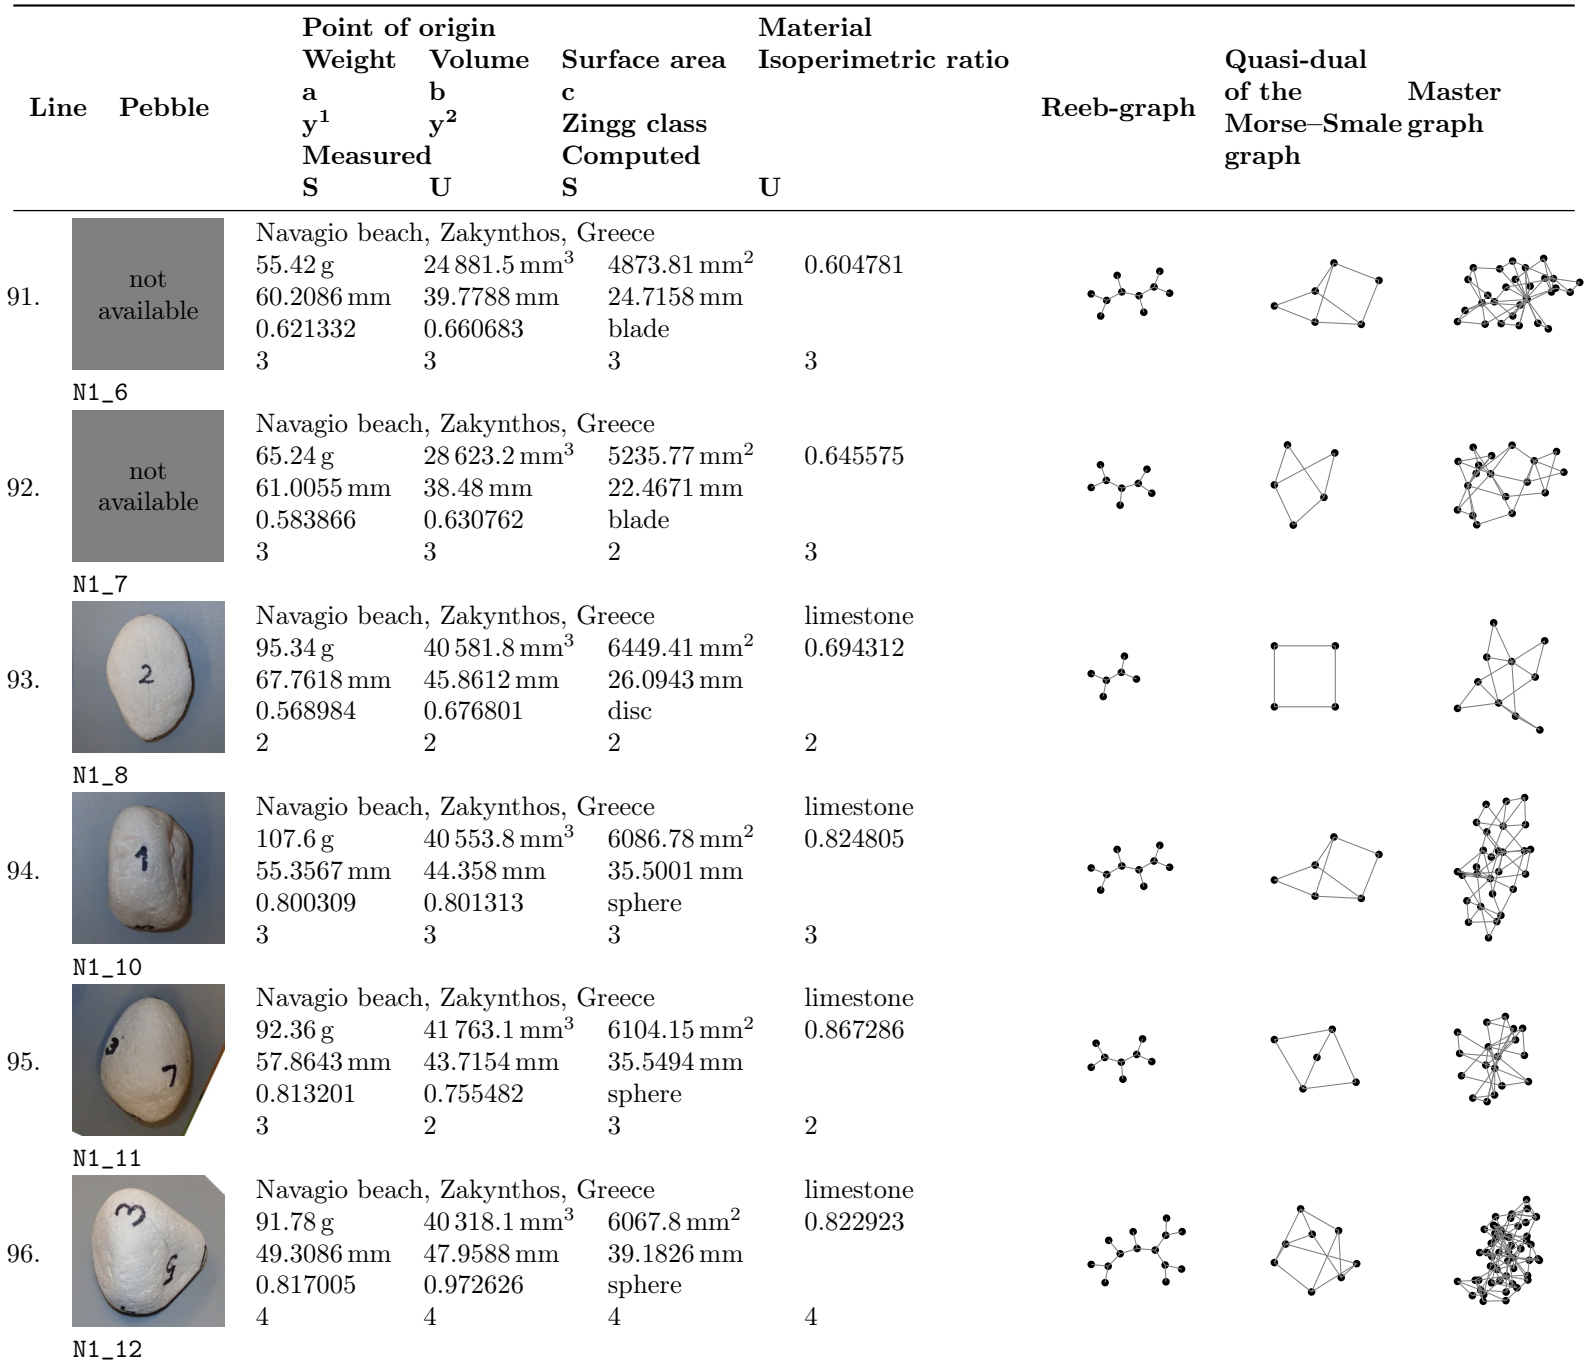   |
|      |                                                                                     | 55.42 g                              | 24 881.5 mm <sup>3</sup> | 4873.81 mm <sup>2</sup>                           |                                      |                                                                                       |                                                                                       |                                                                                       |
|      |                                                                                     | 60.2086 mm                           | 39.7788 mm               | 24.7158 mm                                        |                                      |                                                                                       |                                                                                       |                                                                                       |
|      |                                                                                     | 0.621332                             | 0.660683                 | blade                                             |                                      |                                                                                       |                                                                                       |                                                                                       |
|      | N1_6                                                                                | 3                                    | 3                        | 3                                                 | 3                                    |                                                                                       |                                                                                       |                                                                                       |
| 92.  | 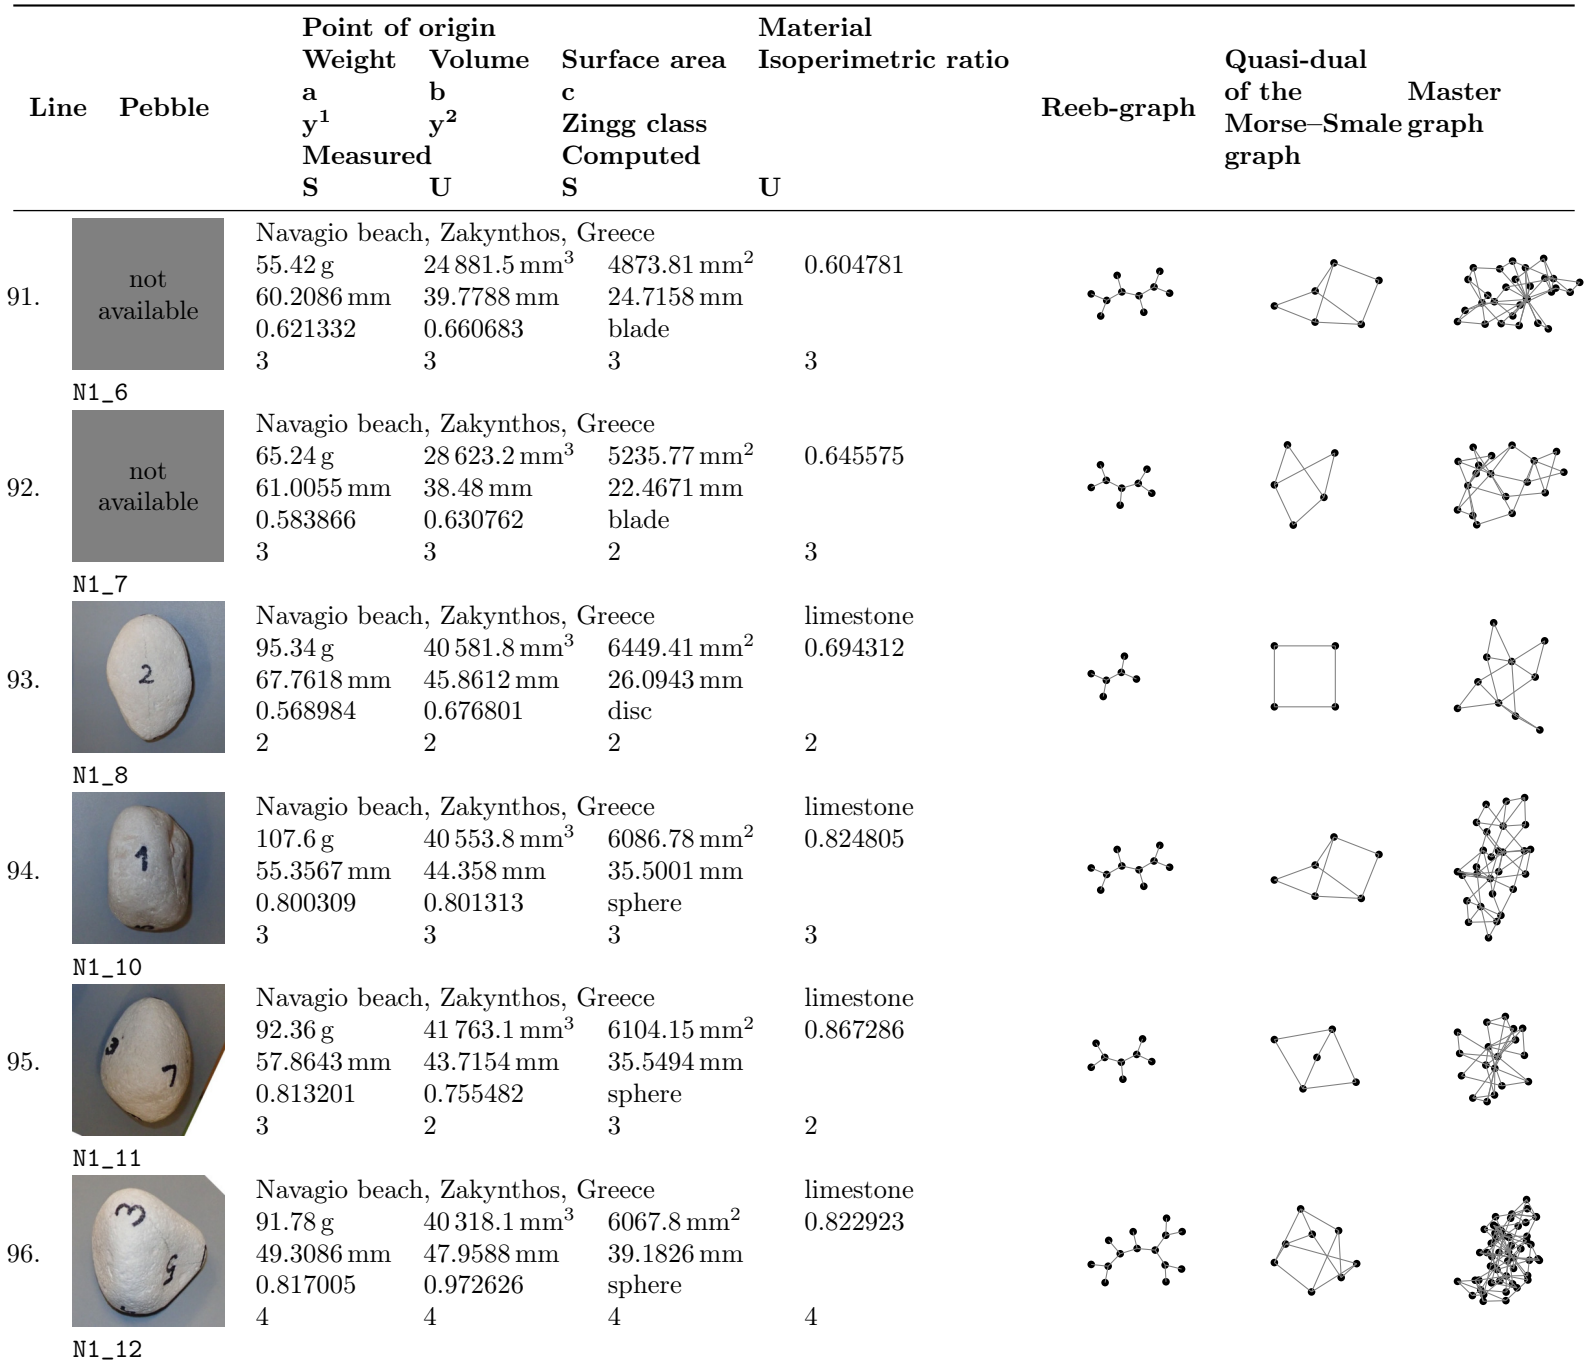   | Navagio beach, Zakynthos, Greece     |                          |                                                   | 0.645575                             | 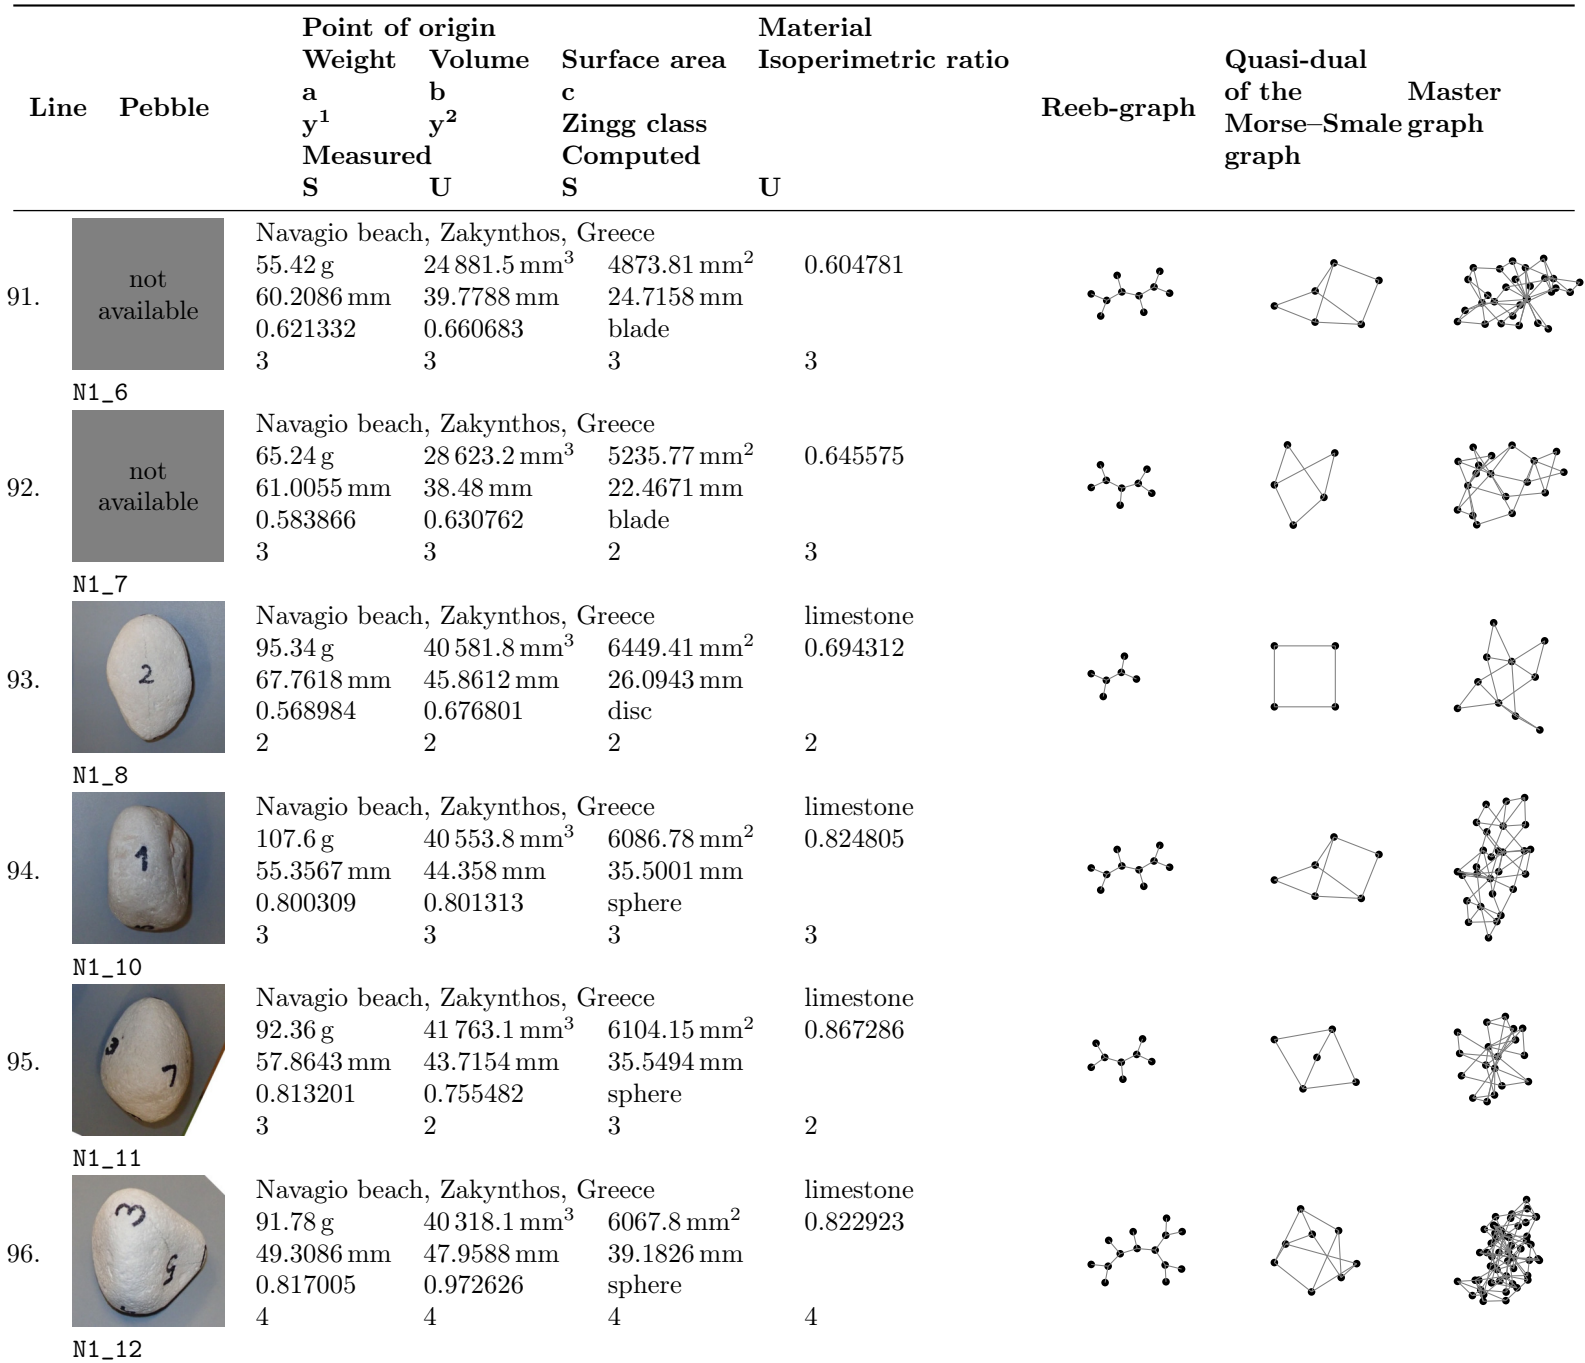   | 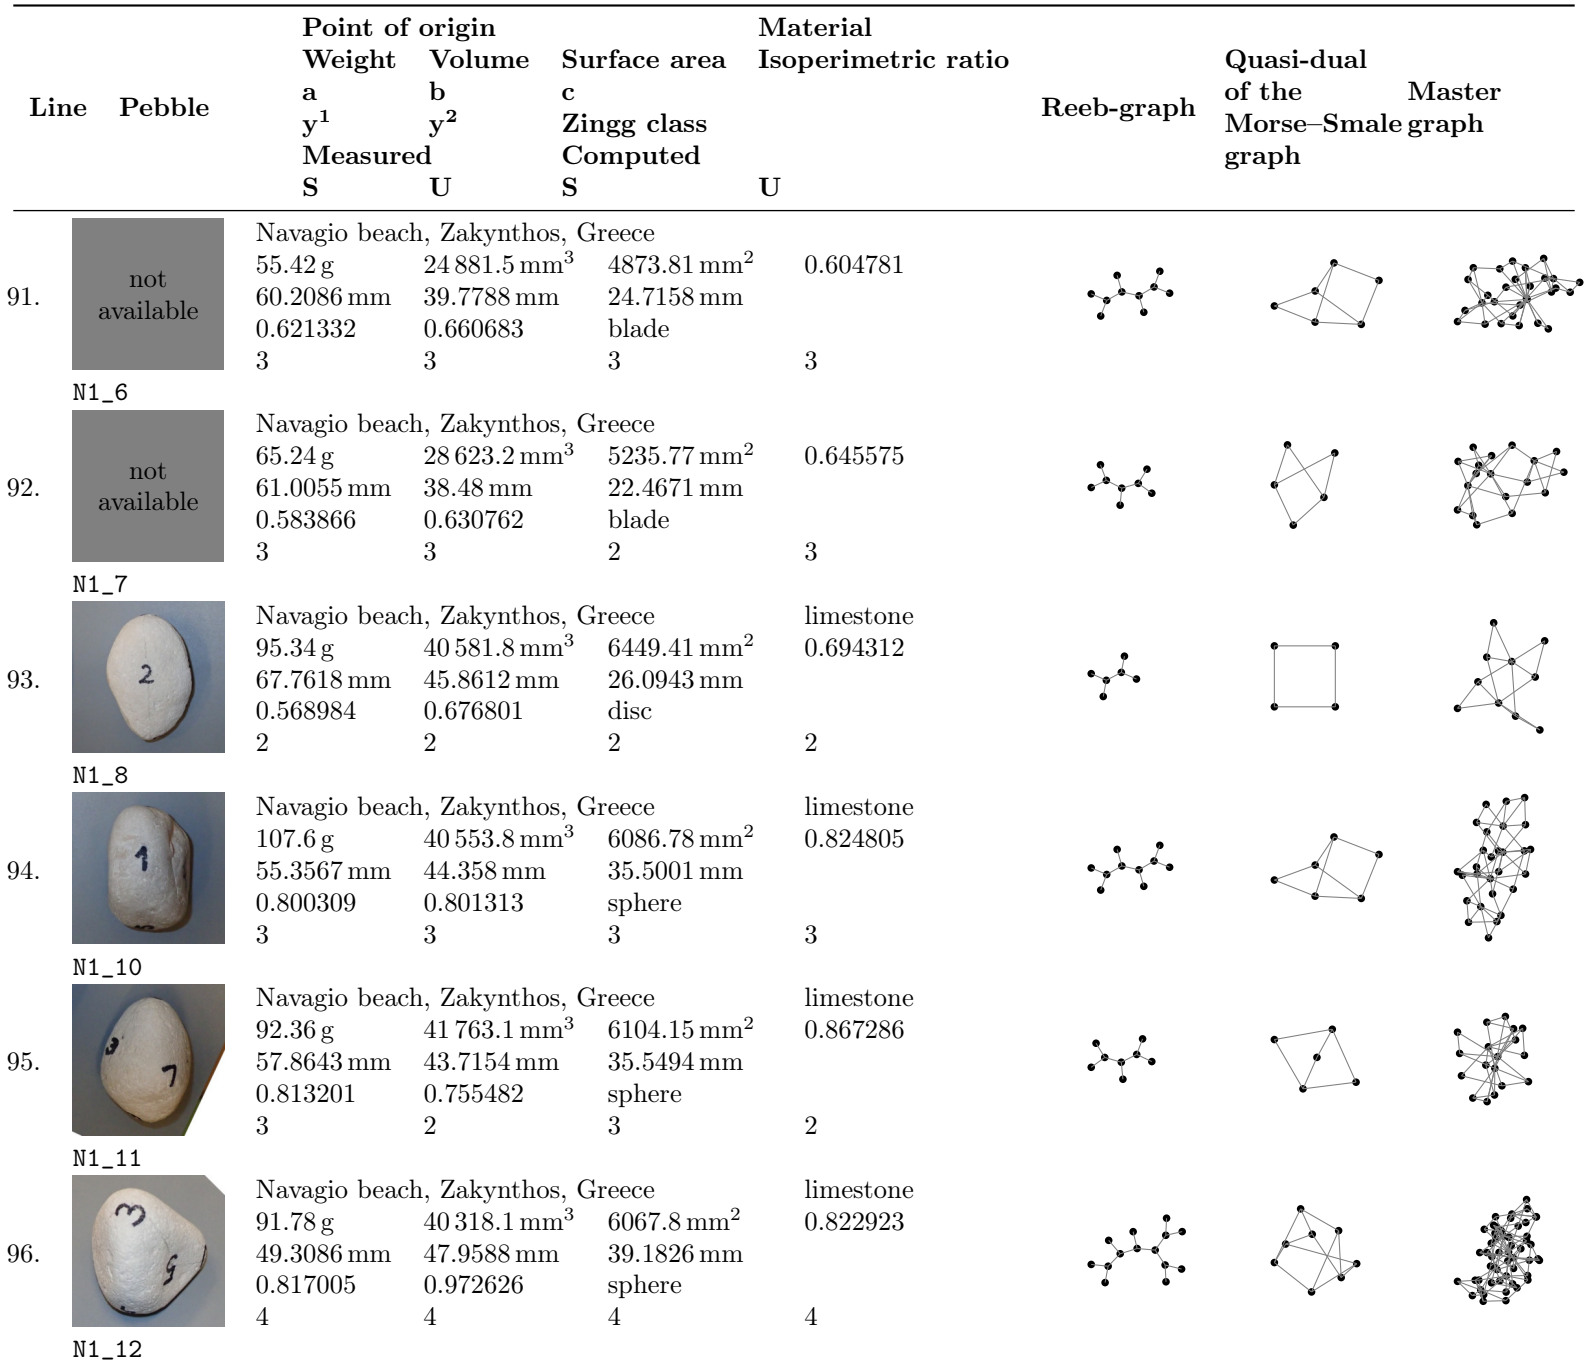   | 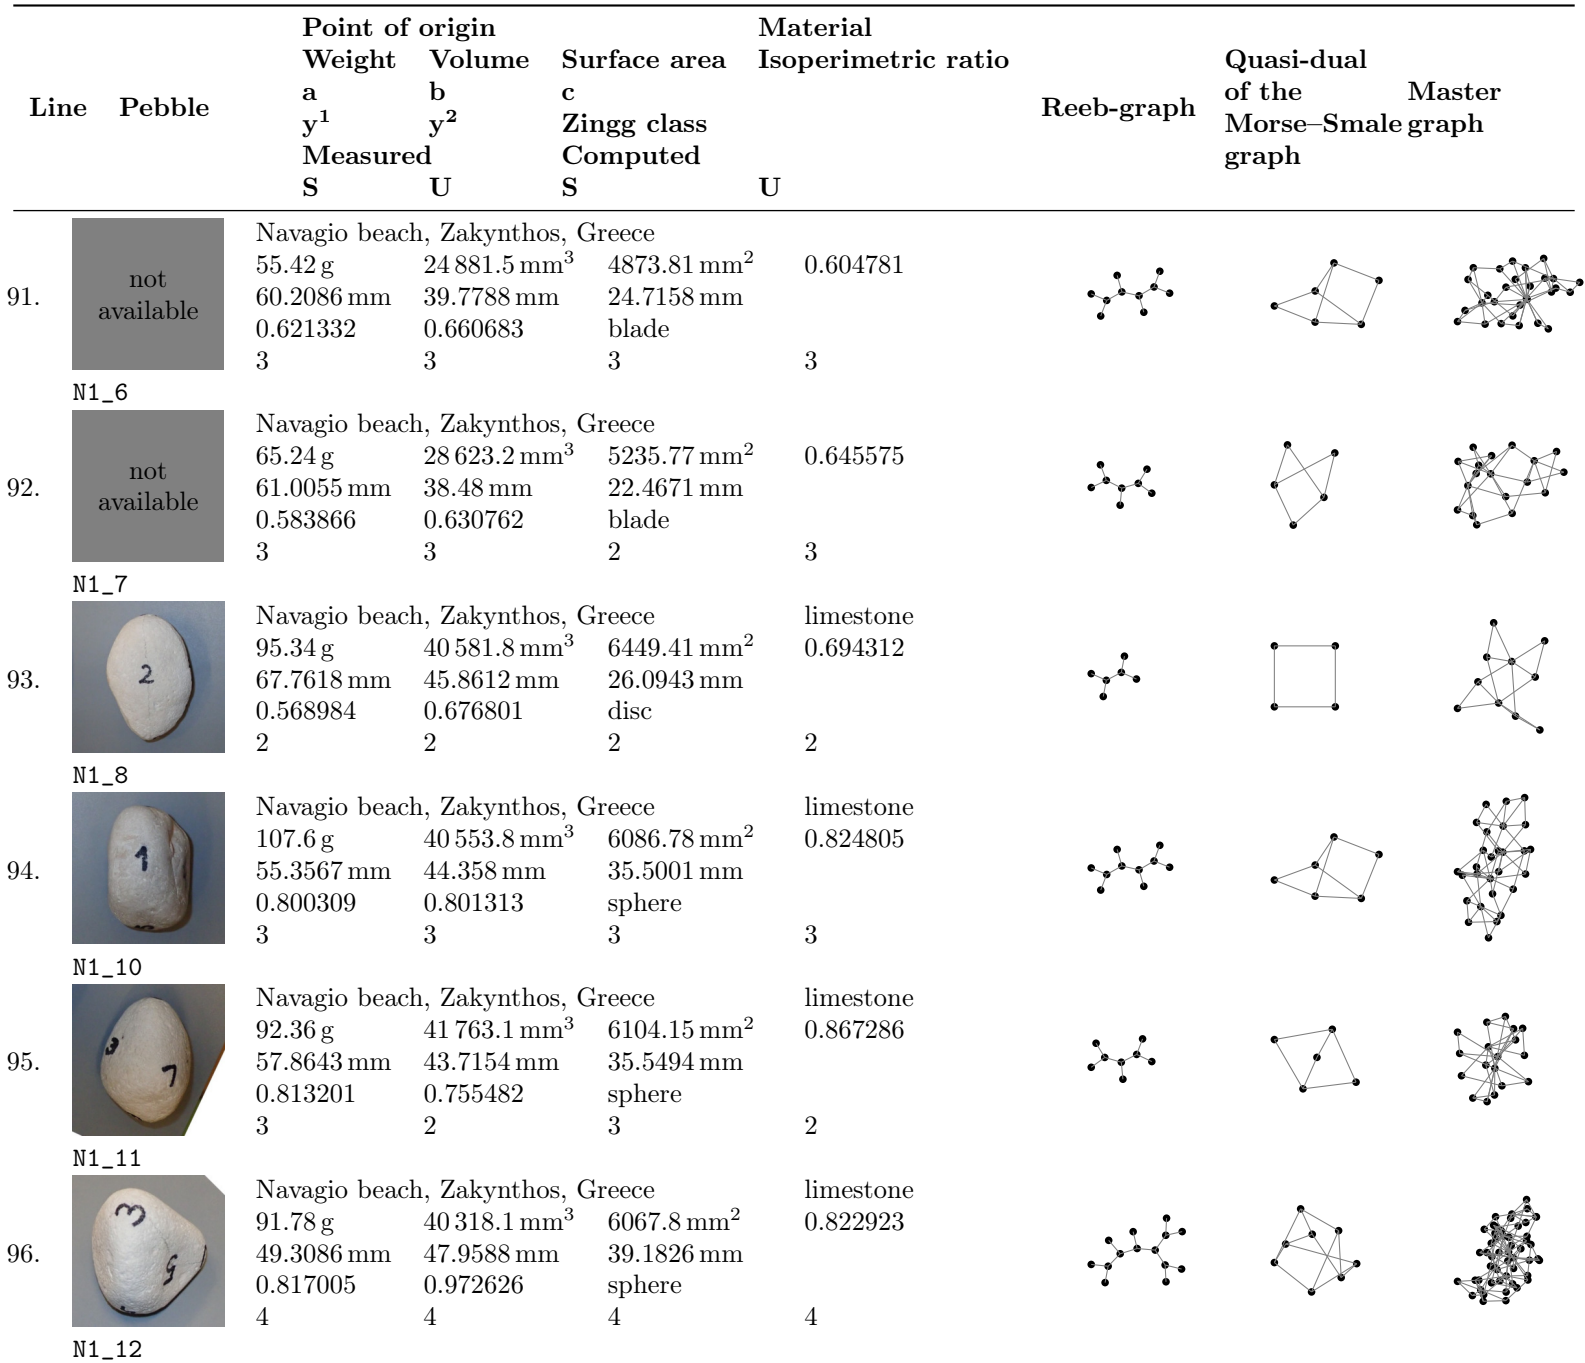   |
|      |                                                                                     | 65.24 g                              | 28 623.2 mm <sup>3</sup> | 5235.77 mm <sup>2</sup>                           |                                      |                                                                                       |                                                                                       |                                                                                       |
|      |                                                                                     | 61.0055 mm                           | 38.48 mm                 | 22.4671 mm                                        |                                      |                                                                                       |                                                                                       |                                                                                       |
|      |                                                                                     | 0.583866                             | 0.630762                 | blade                                             |                                      |                                                                                       |                                                                                       |                                                                                       |
|      | N1_7                                                                                | 3                                    | 3                        | 2                                                 | 3                                    |                                                                                       |                                                                                       |                                                                                       |
| 93.  | 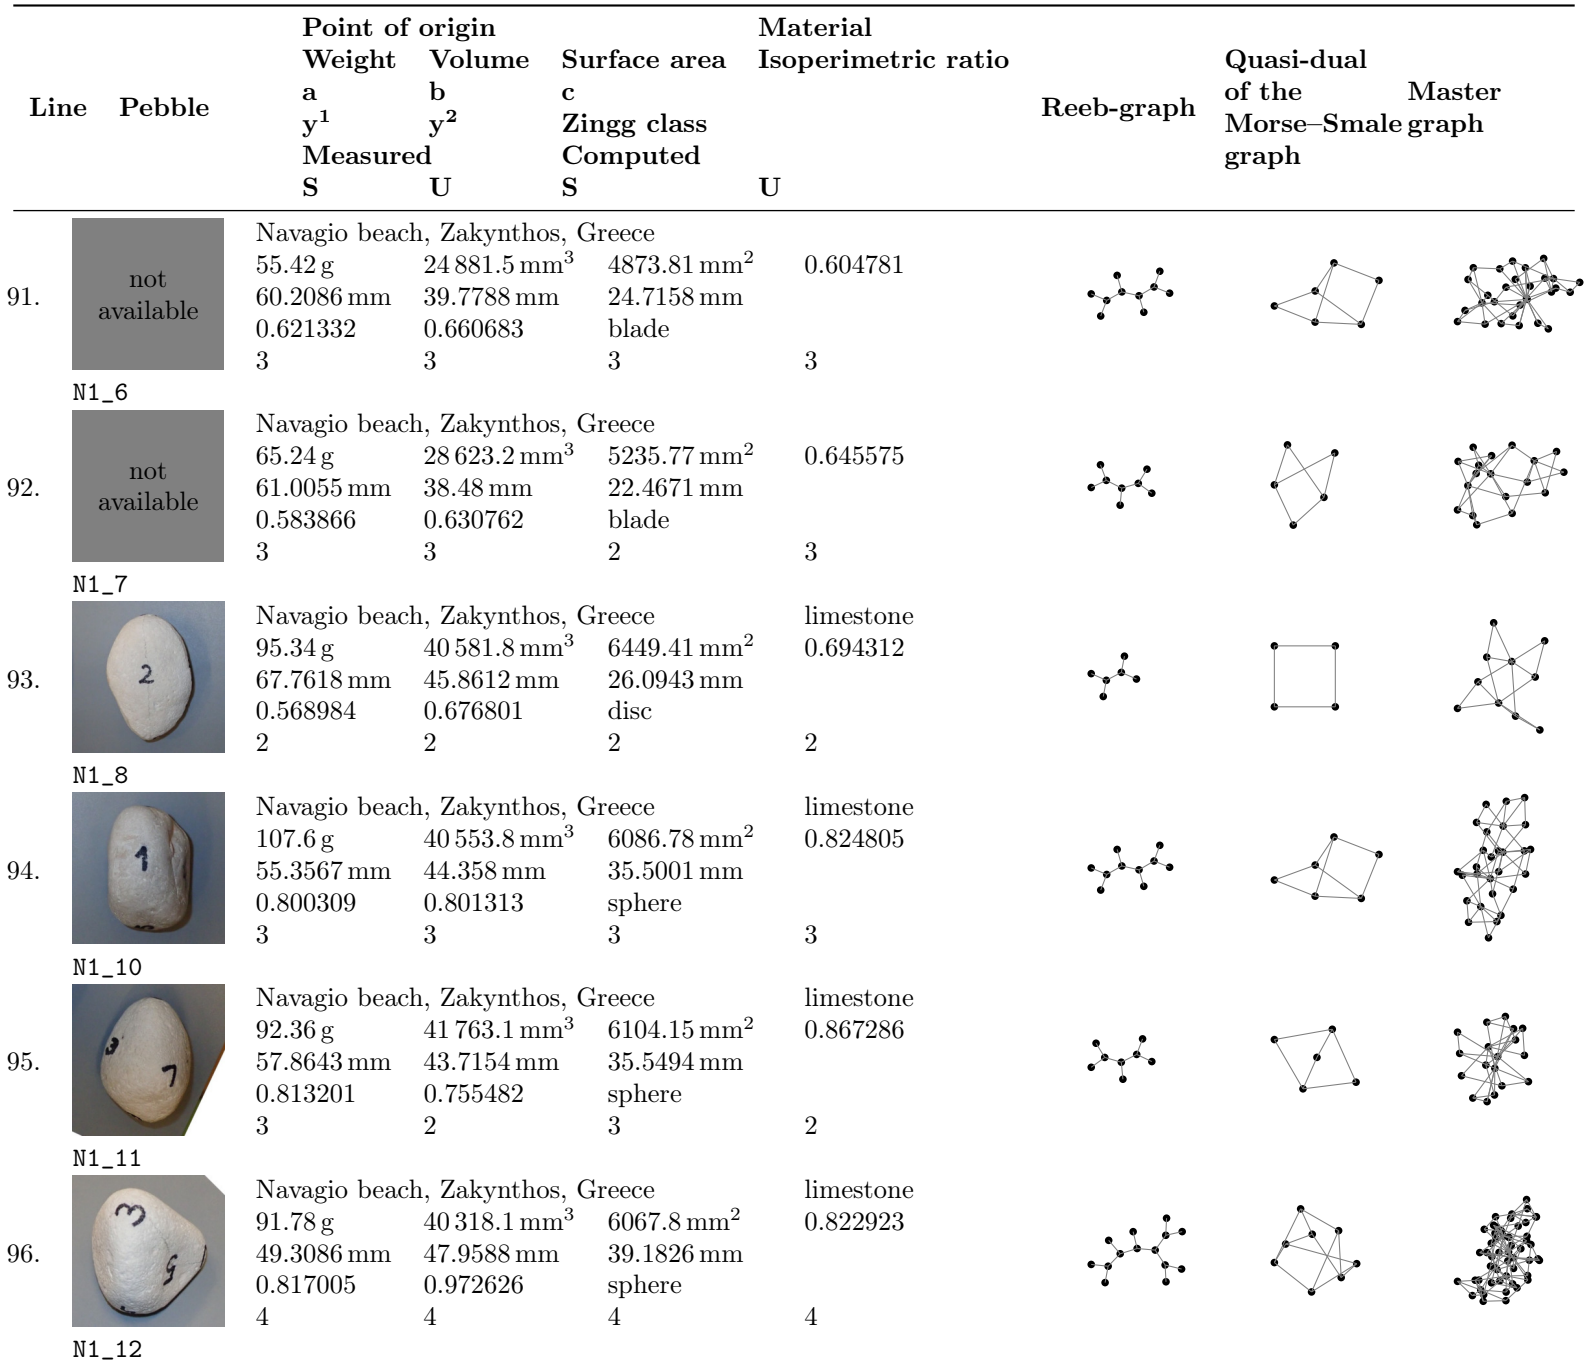   | Navagio beach, Zakynthos, Greece     |                          |                                                   | limestone<br>0.694312                | 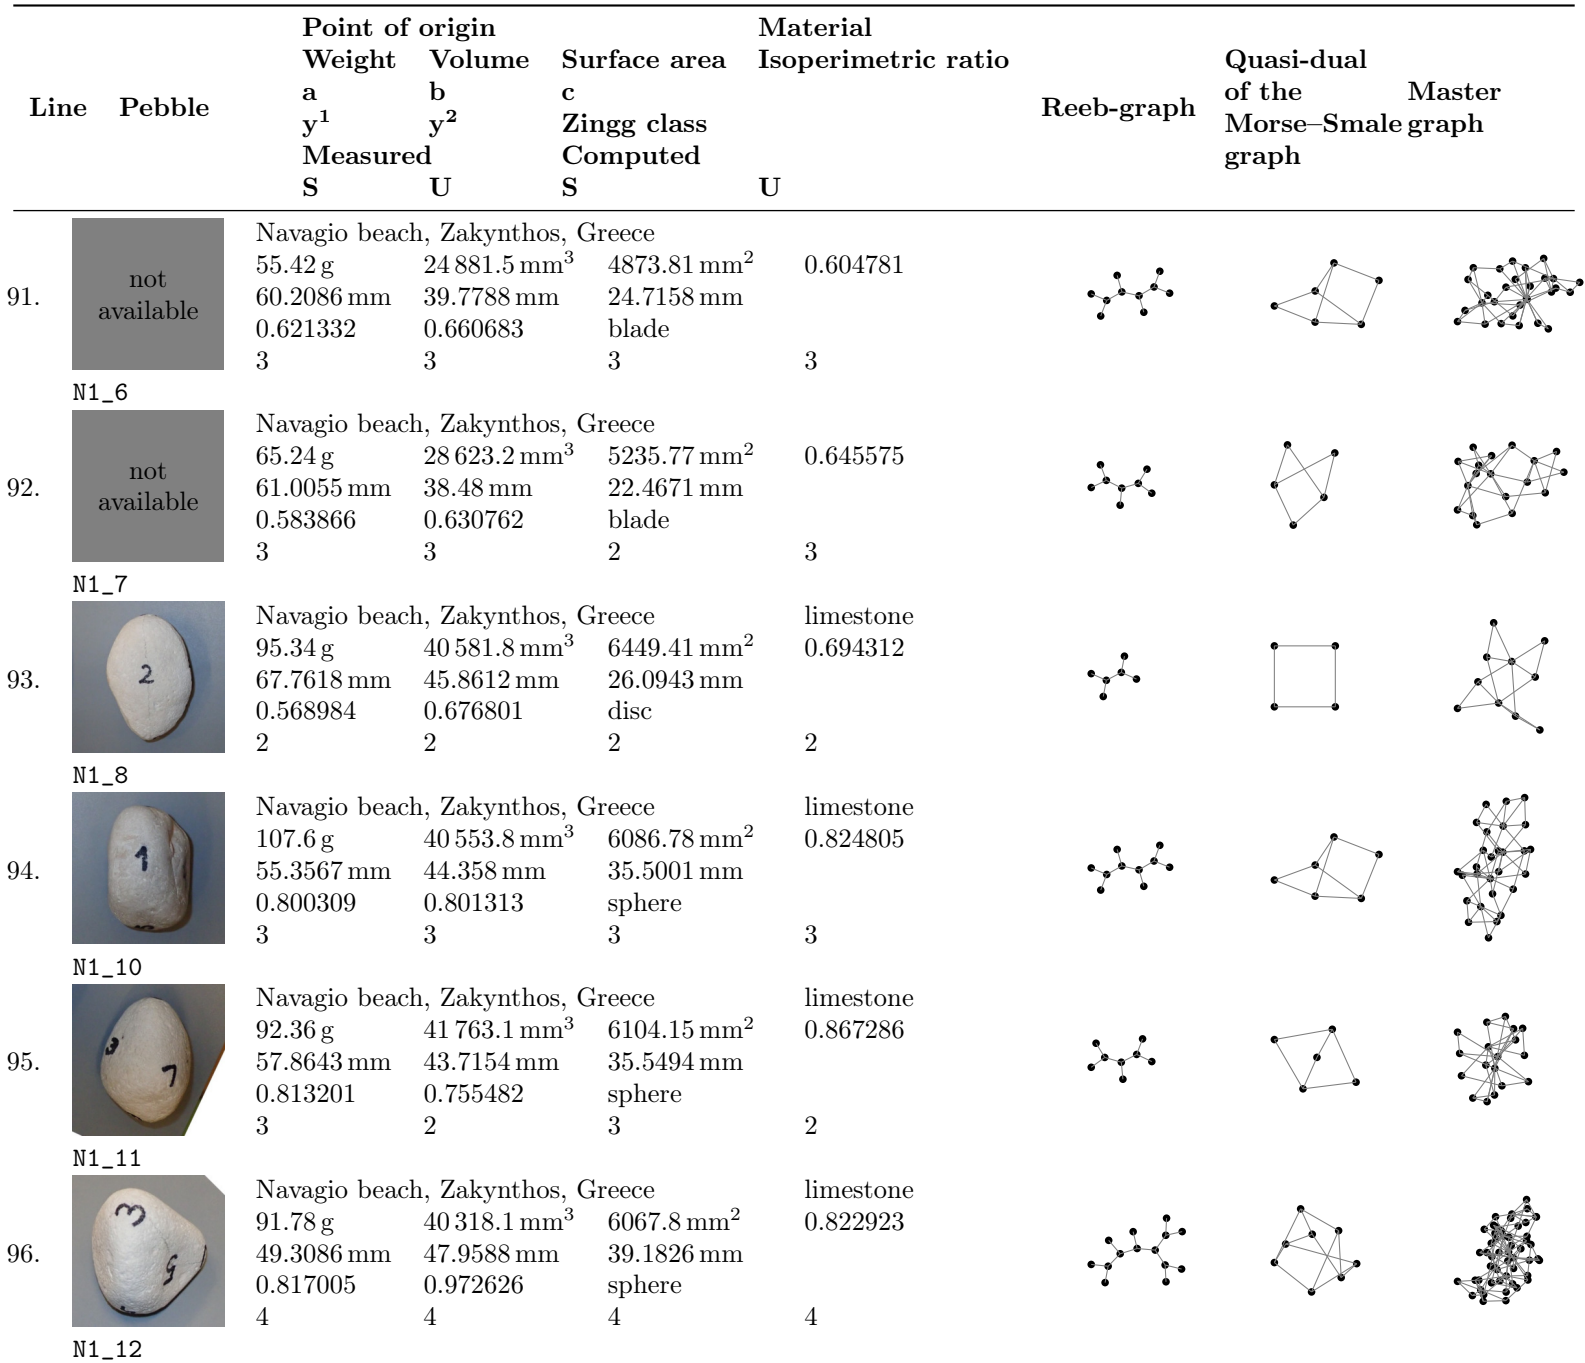   | 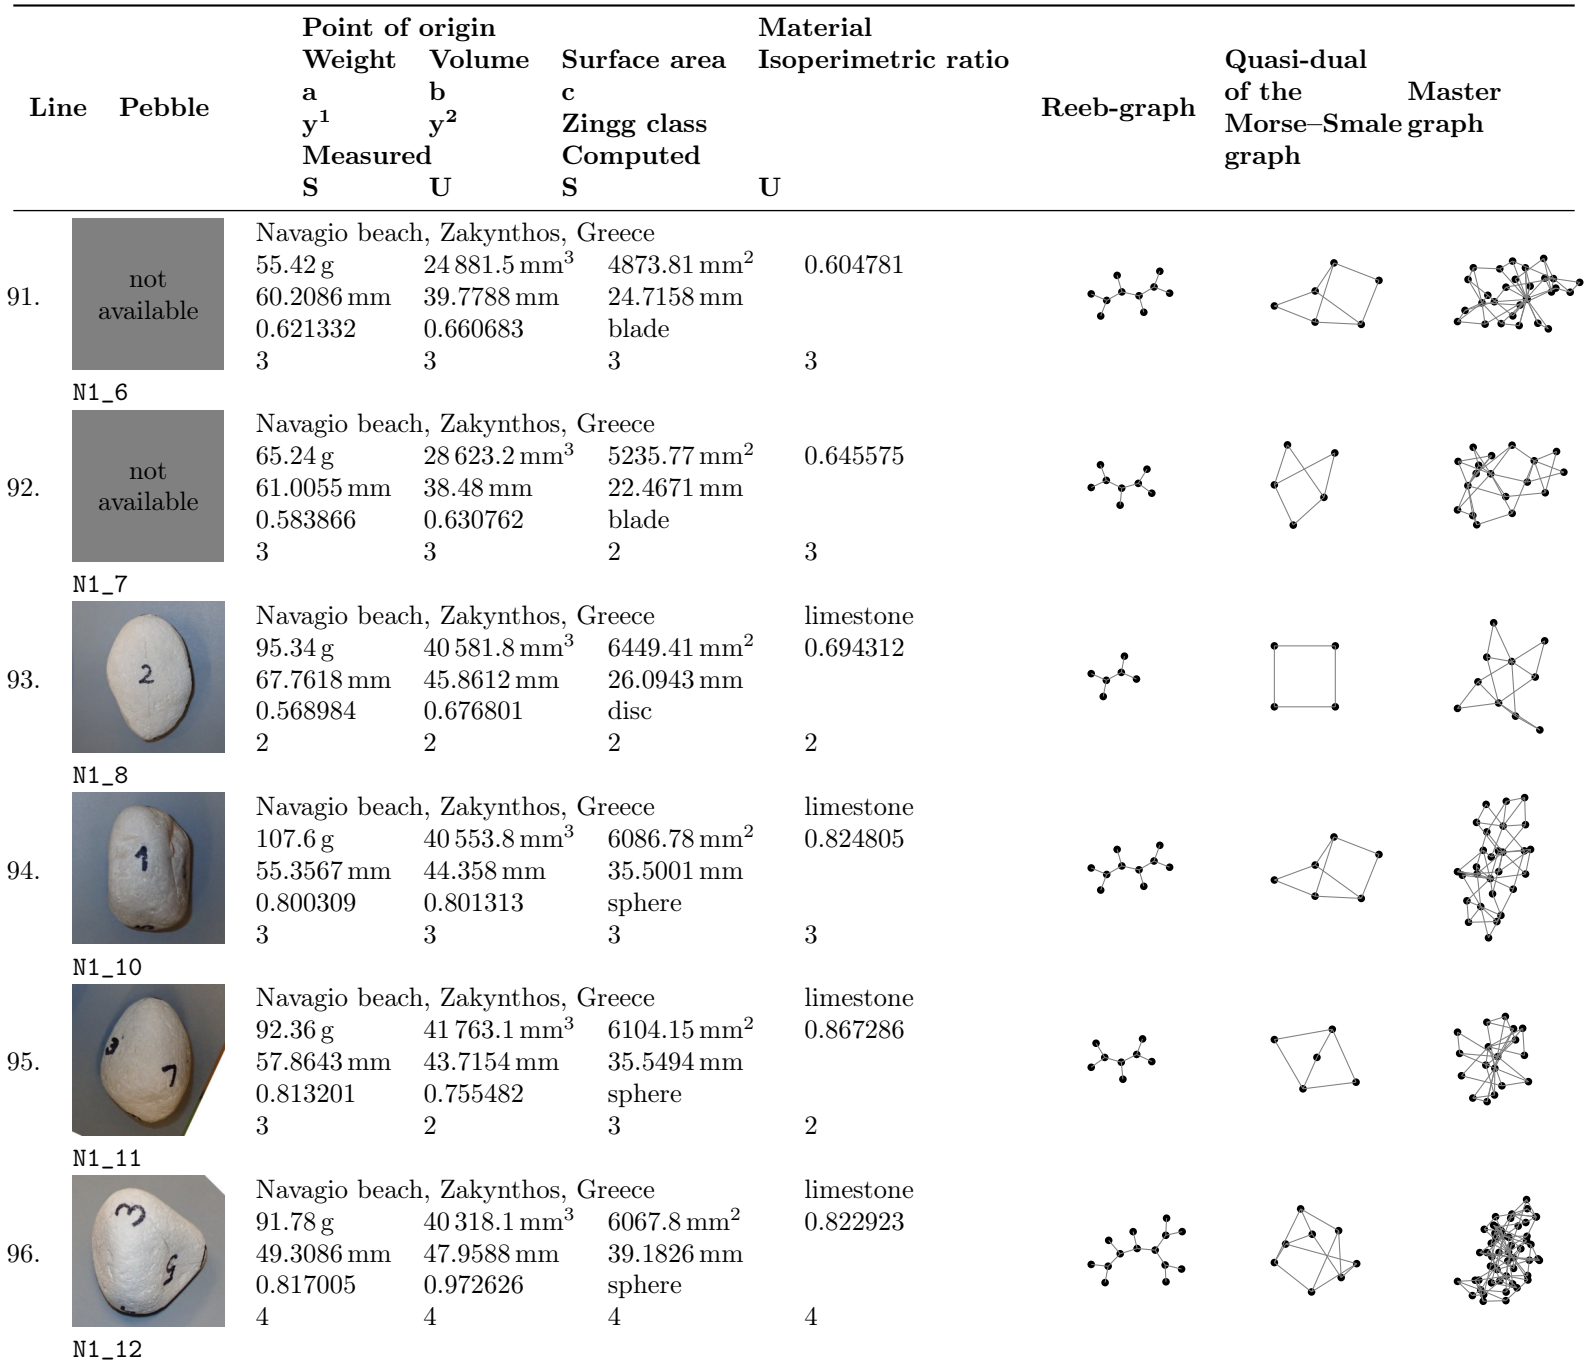   | 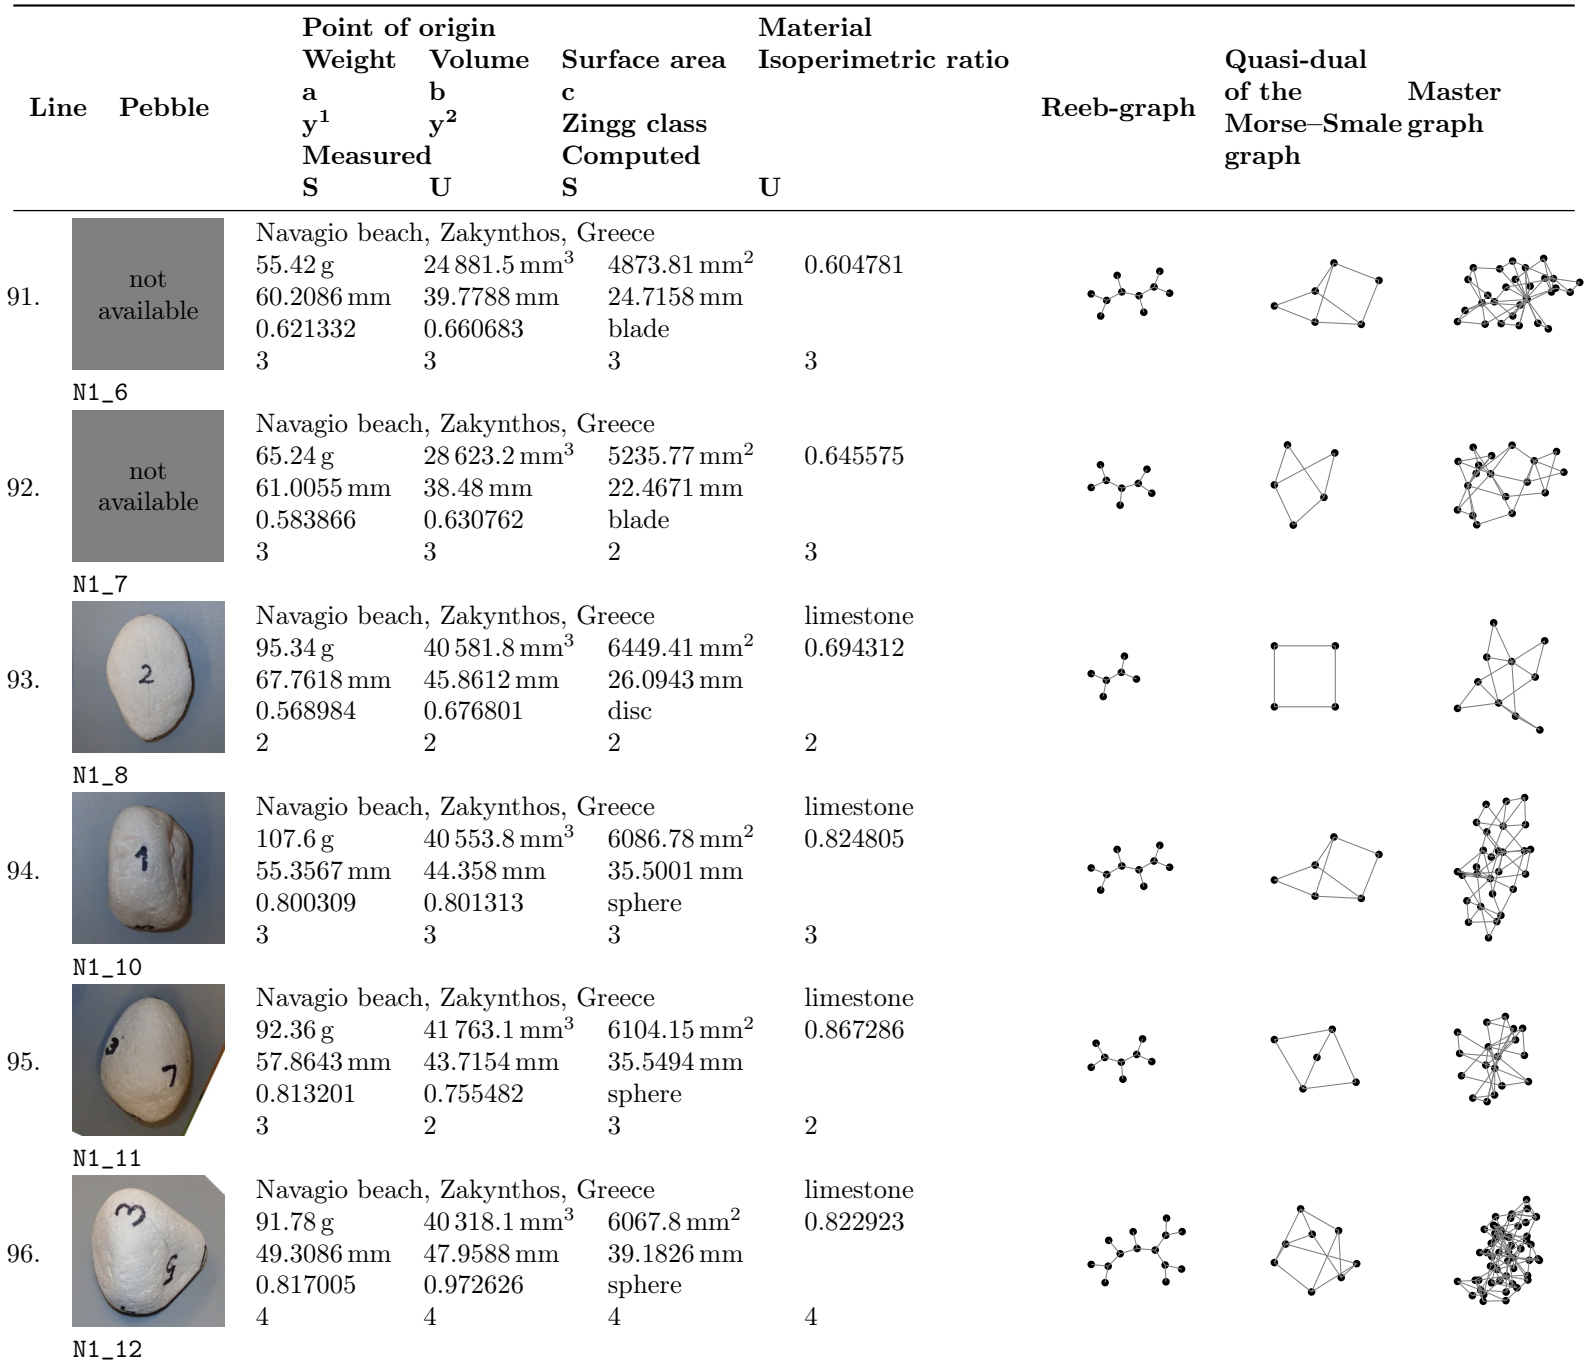   |
|      |                                                                                     | 95.34 g                              | 40 581.8 mm <sup>3</sup> | 6449.41 mm <sup>2</sup>                           |                                      |                                                                                       |                                                                                       |                                                                                       |
|      |                                                                                     | 67.7618 mm                           | 45.8612 mm               | 26.0943 mm                                        |                                      |                                                                                       |                                                                                       |                                                                                       |
|      |                                                                                     | 0.568984                             | 0.676801                 | disc                                              |                                      |                                                                                       |                                                                                       |                                                                                       |
|      | N1_8                                                                                | 2                                    | 2                        | 2                                                 | 2                                    |                                                                                       |                                                                                       |                                                                                       |
| 94.  | 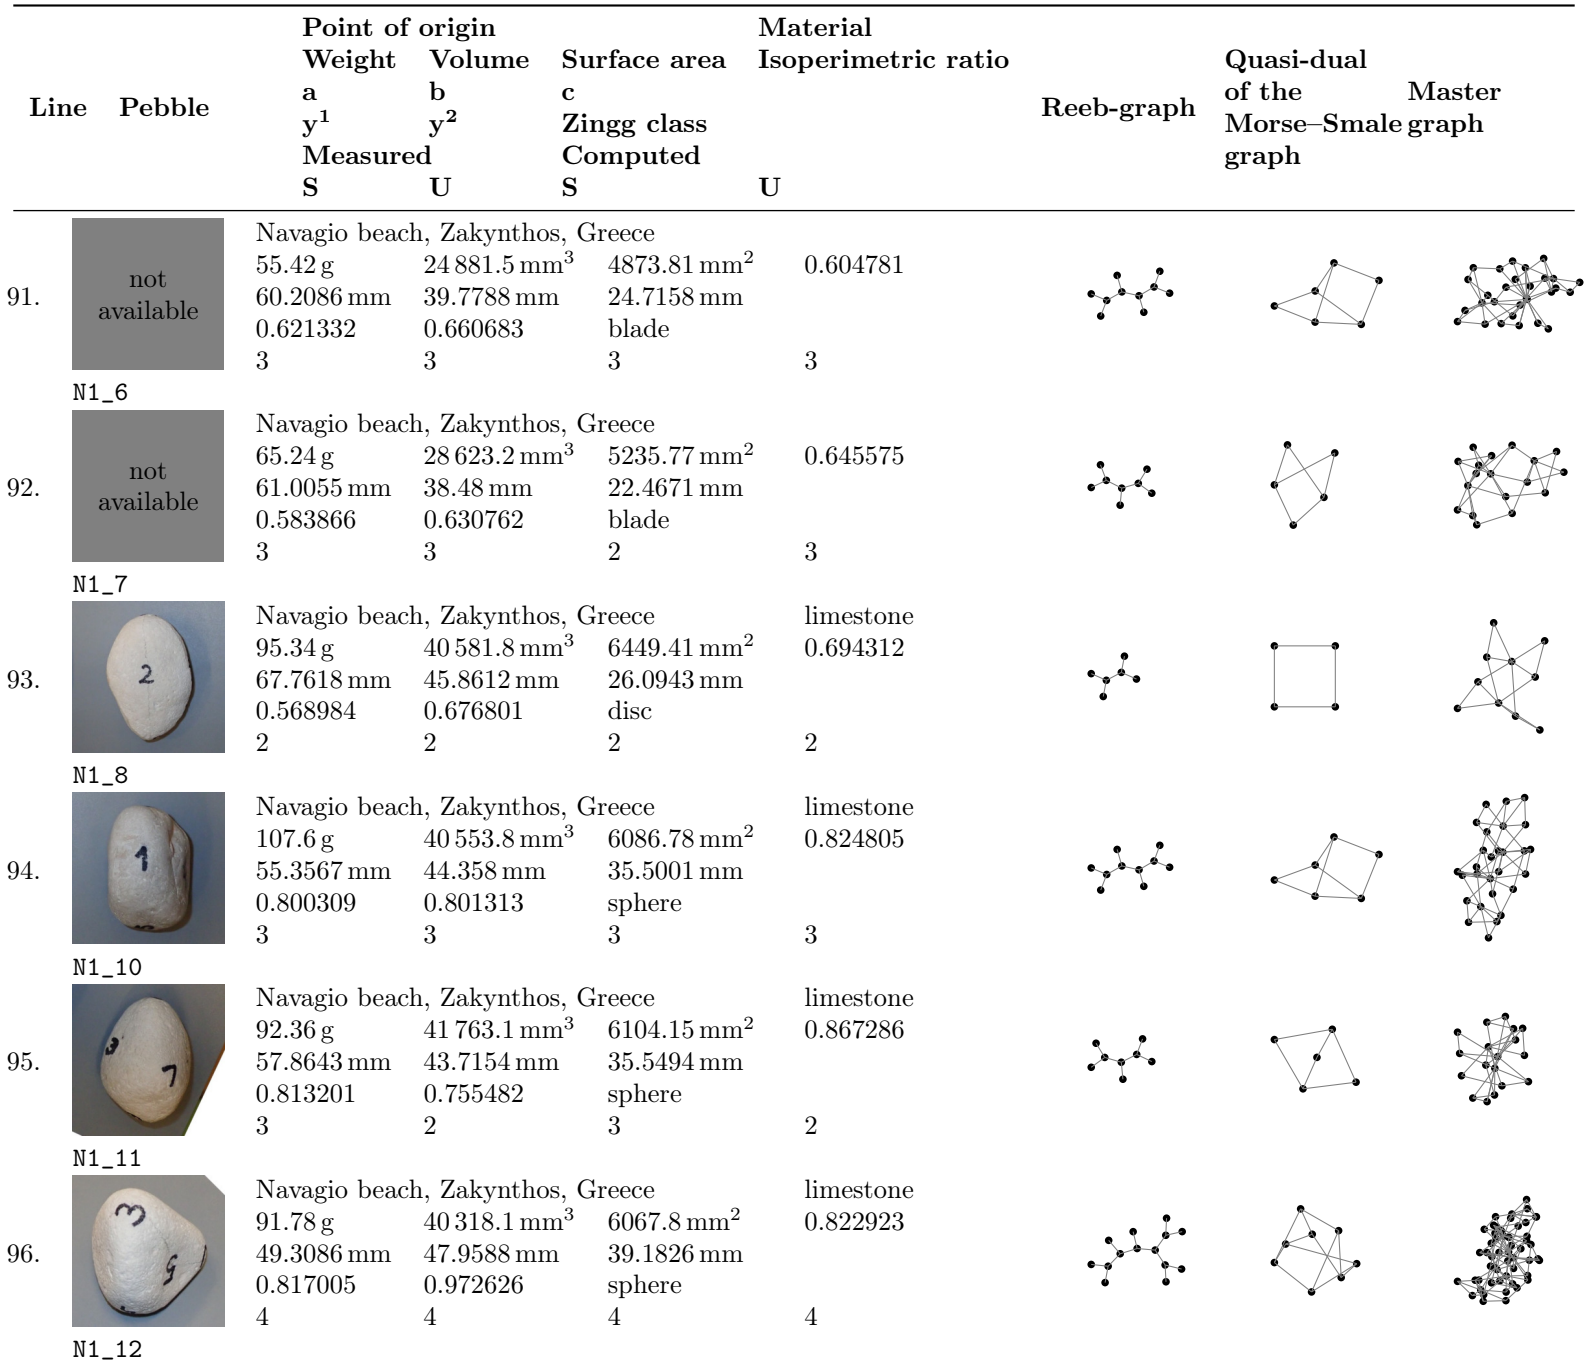  | Navagio beach, Zakynthos, Greece     |                          |                                                   | limestone<br>0.824805                | 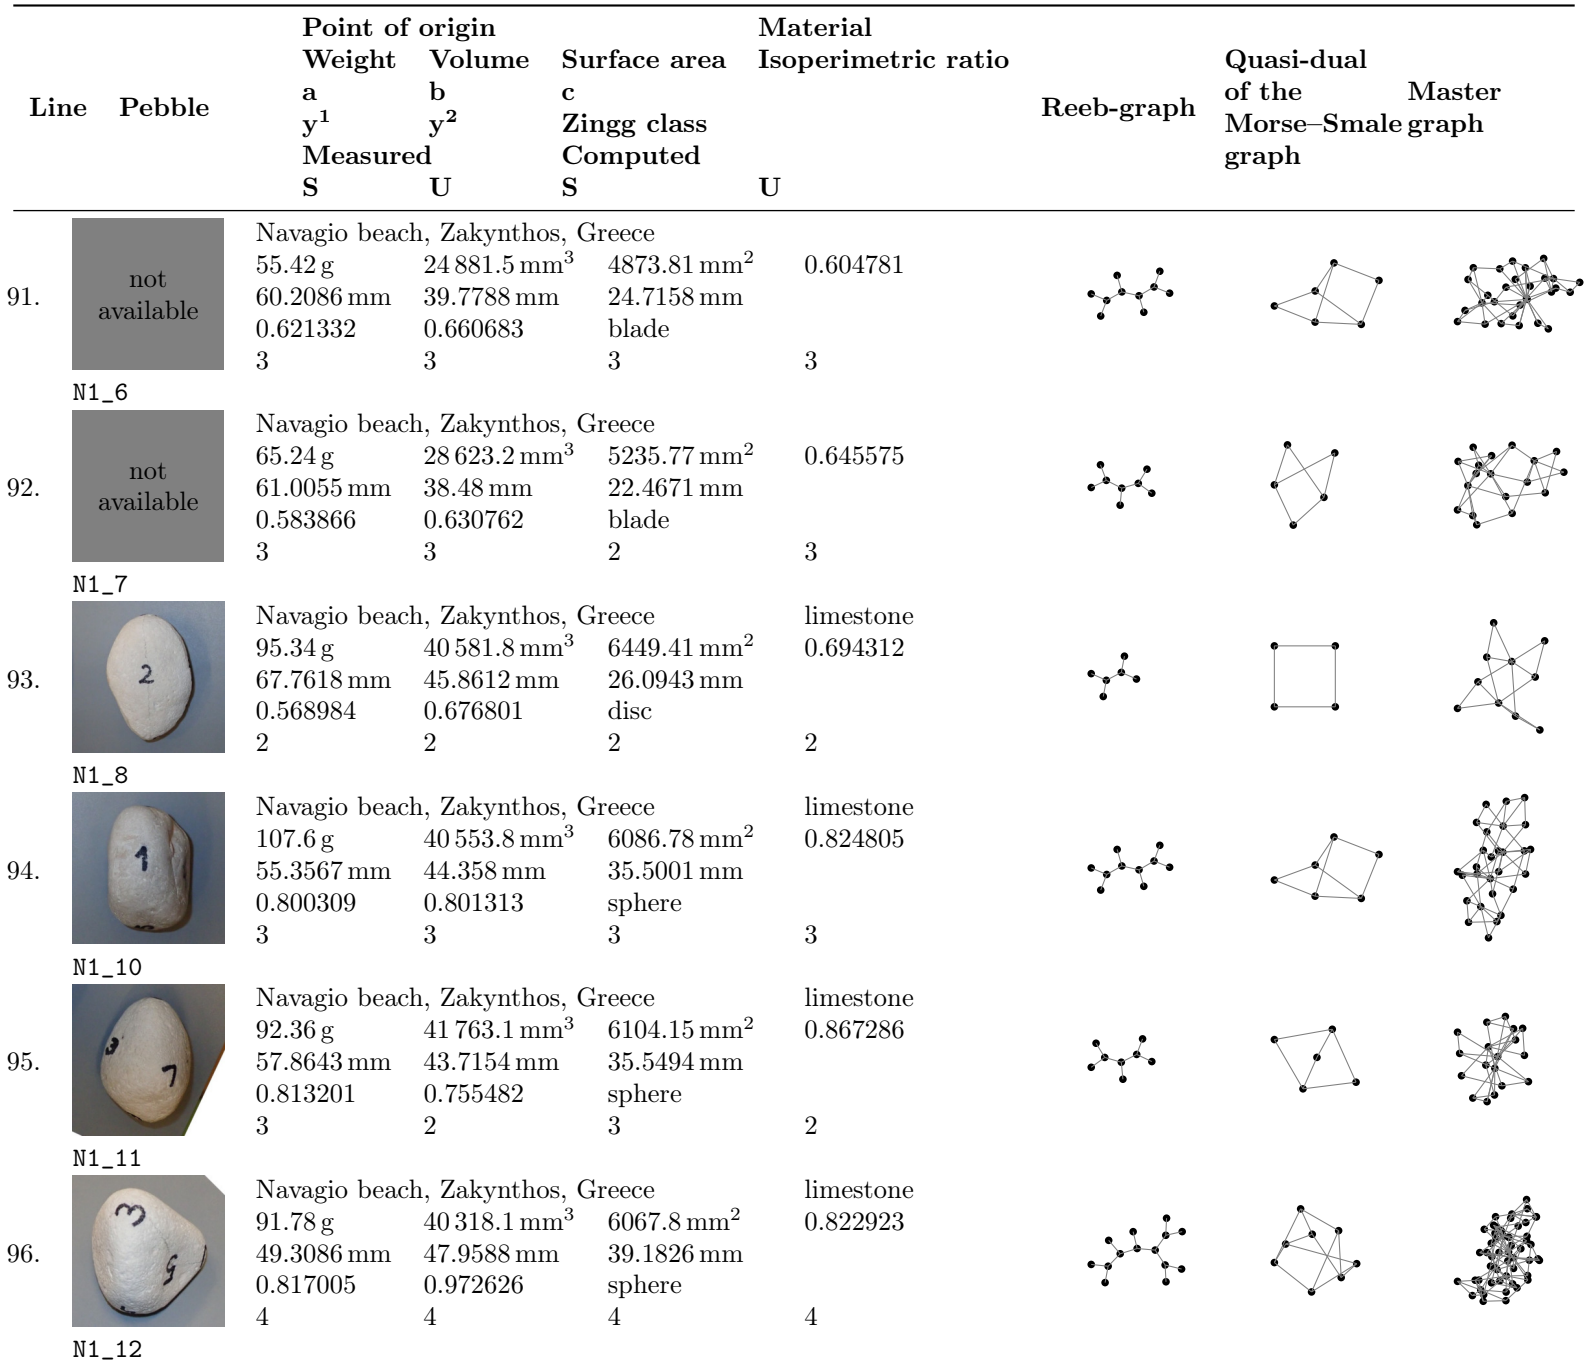  | 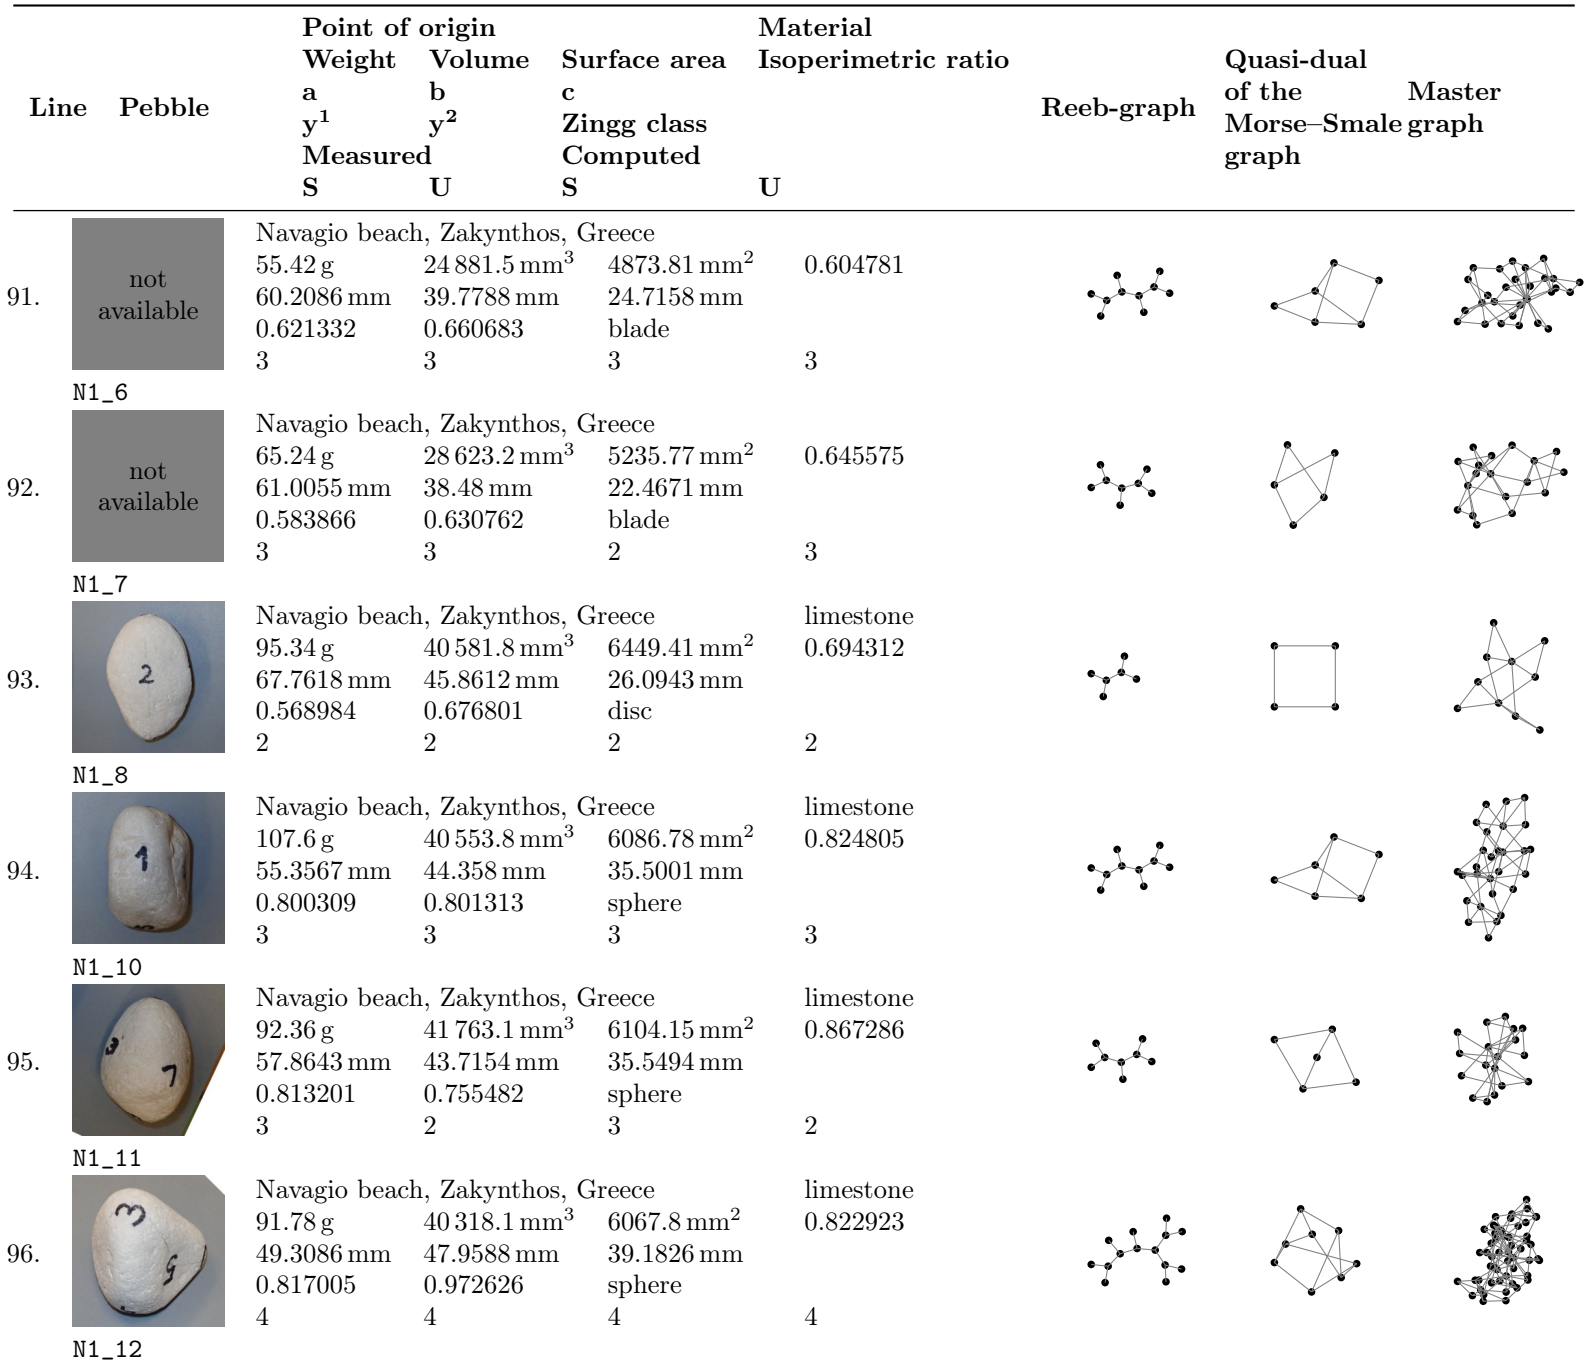  | 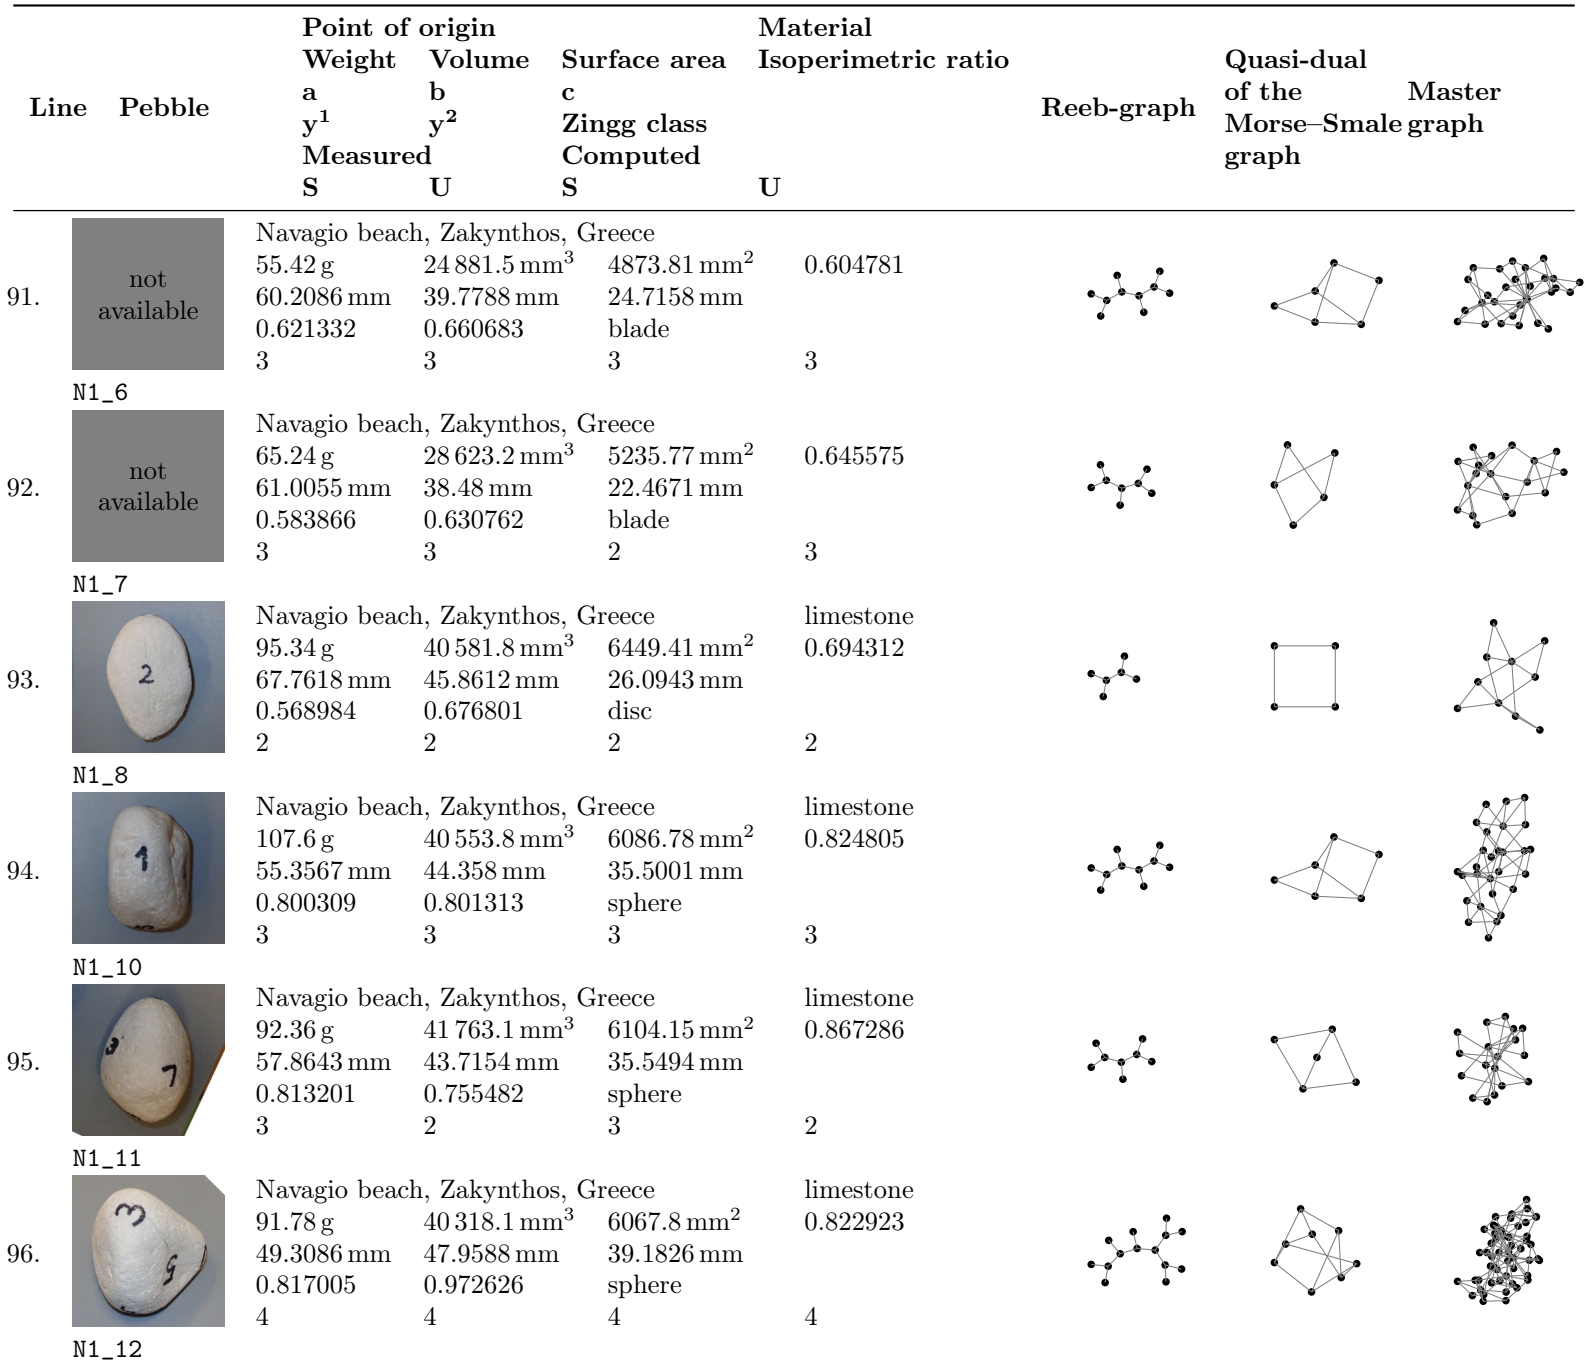  |
|      |                                                                                     | 107.6 g                              | 40 553.8 mm <sup>3</sup> | 6086.78 mm <sup>2</sup>                           |                                      |                                                                                       |                                                                                       |                                                                                       |
|      |                                                                                     | 55.3567 mm                           | 44.358 mm                | 35.5001 mm                                        |                                      |                                                                                       |                                                                                       |                                                                                       |
|      |                                                                                     | 0.800309                             | 0.801313                 | sphere                                            |                                      |                                                                                       |                                                                                       |                                                                                       |
|      | N1_10                                                                               | 3                                    | 3                        | 3                                                 | 3                                    |                                                                                       |                                                                                       |                                                                                       |
| 95.  | 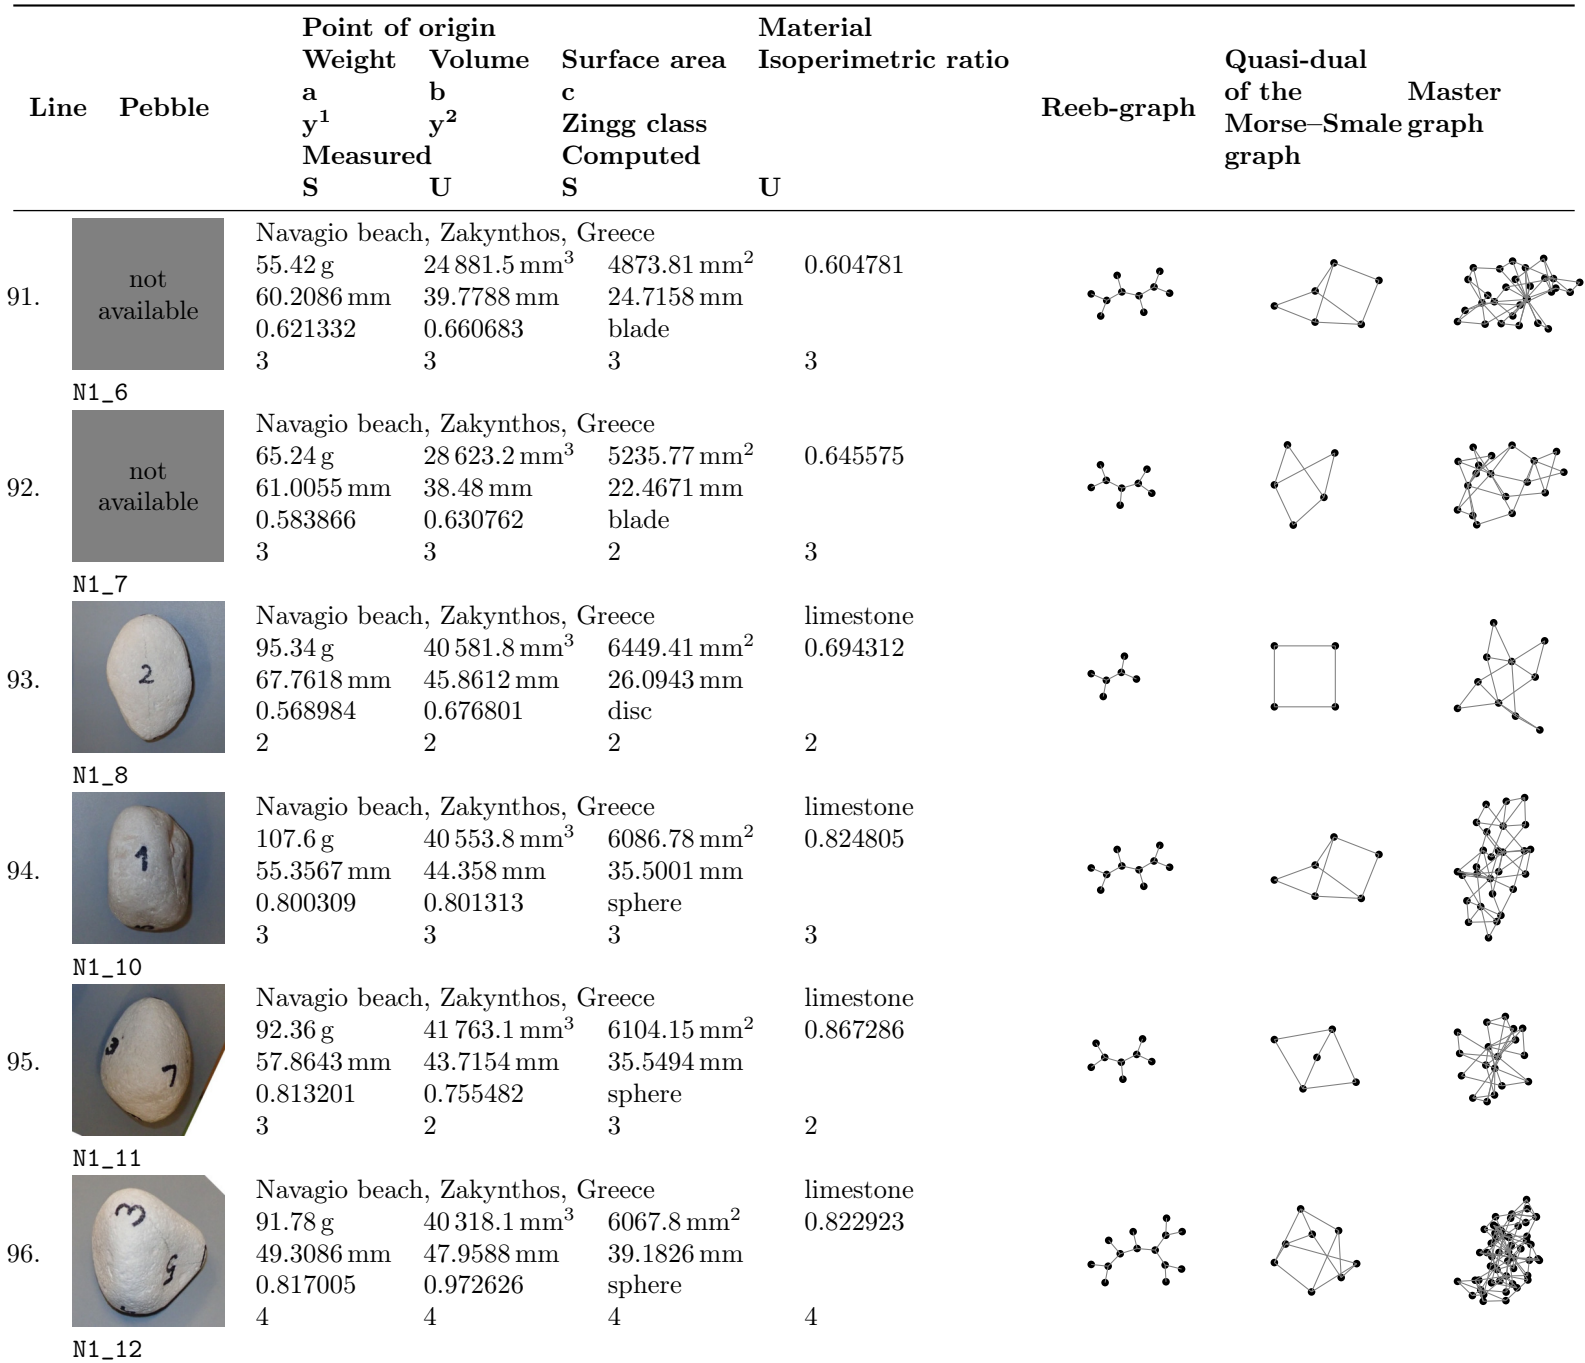 | Navagio beach, Zakynthos, Greece     |                          |                                                   | limestone<br>0.867286                | 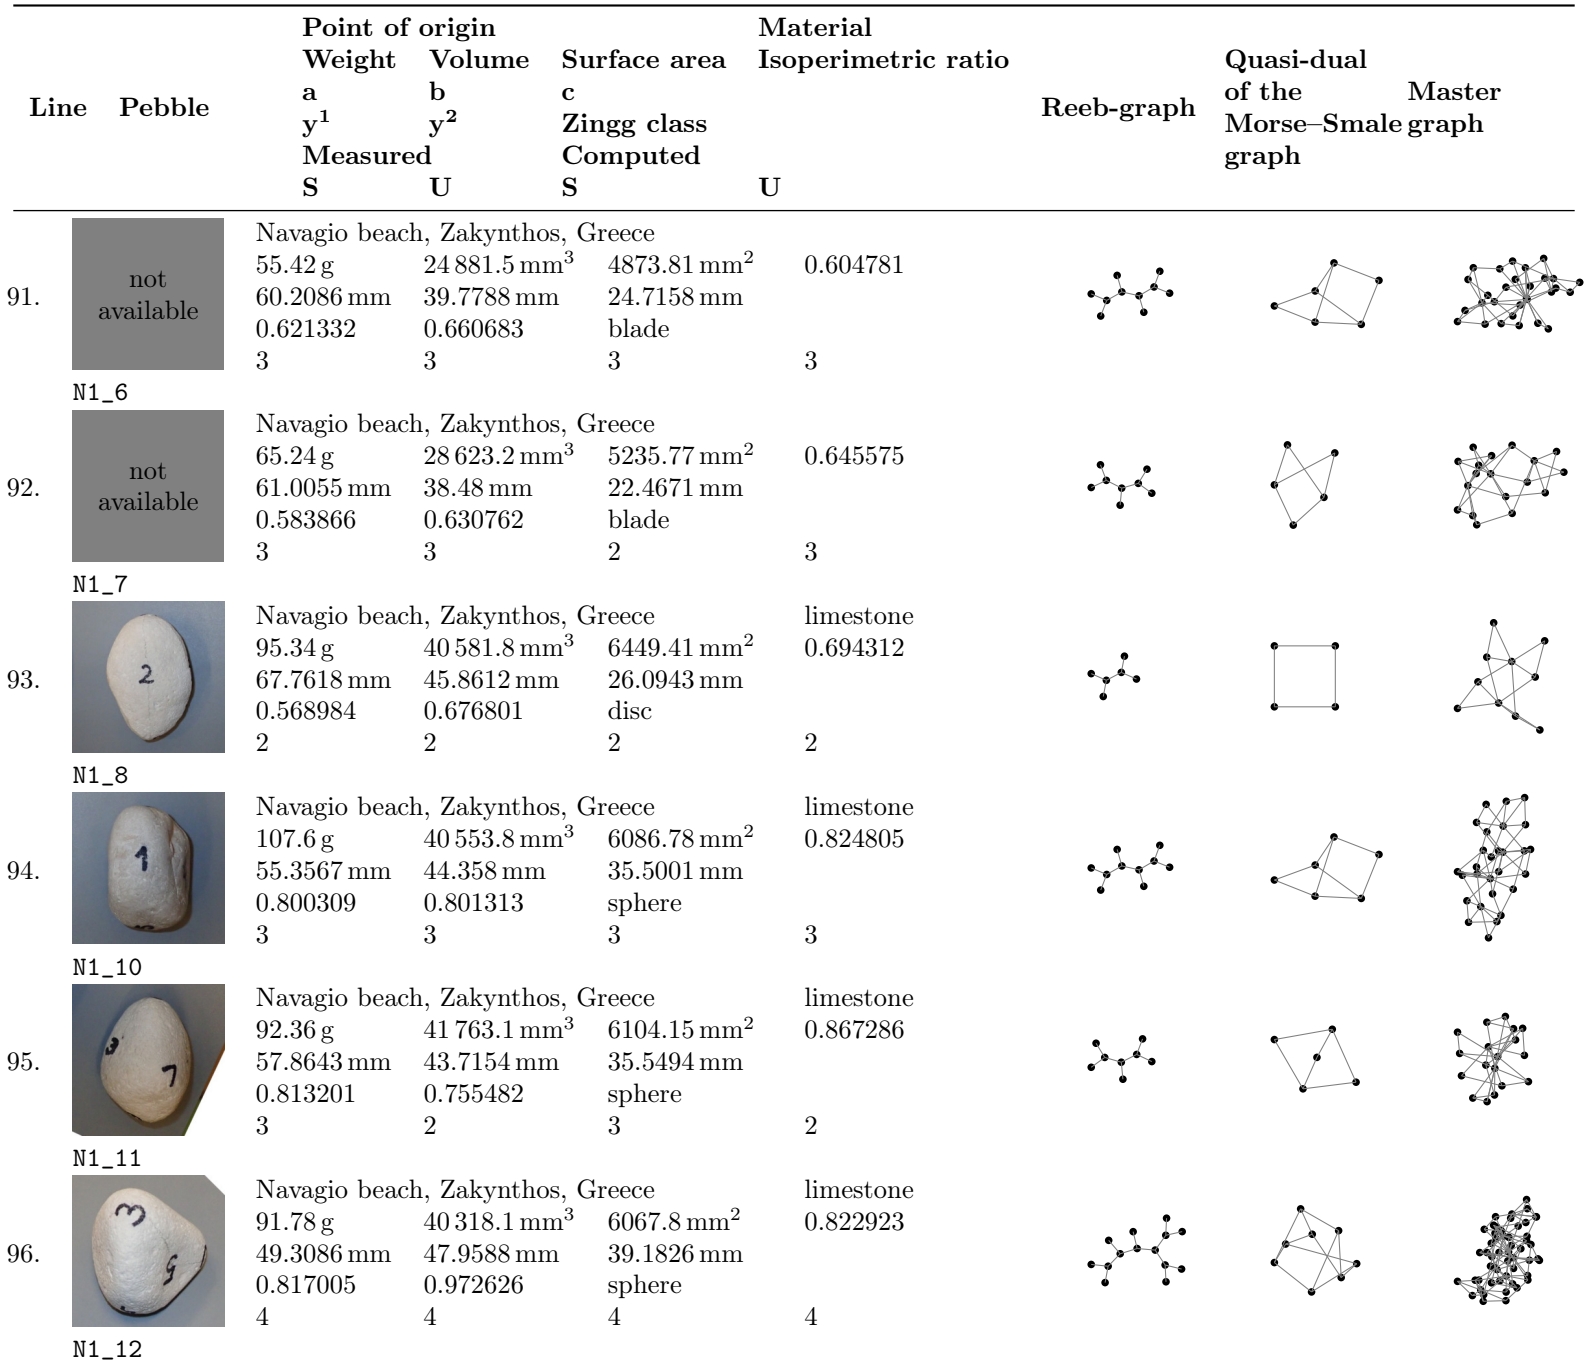 | 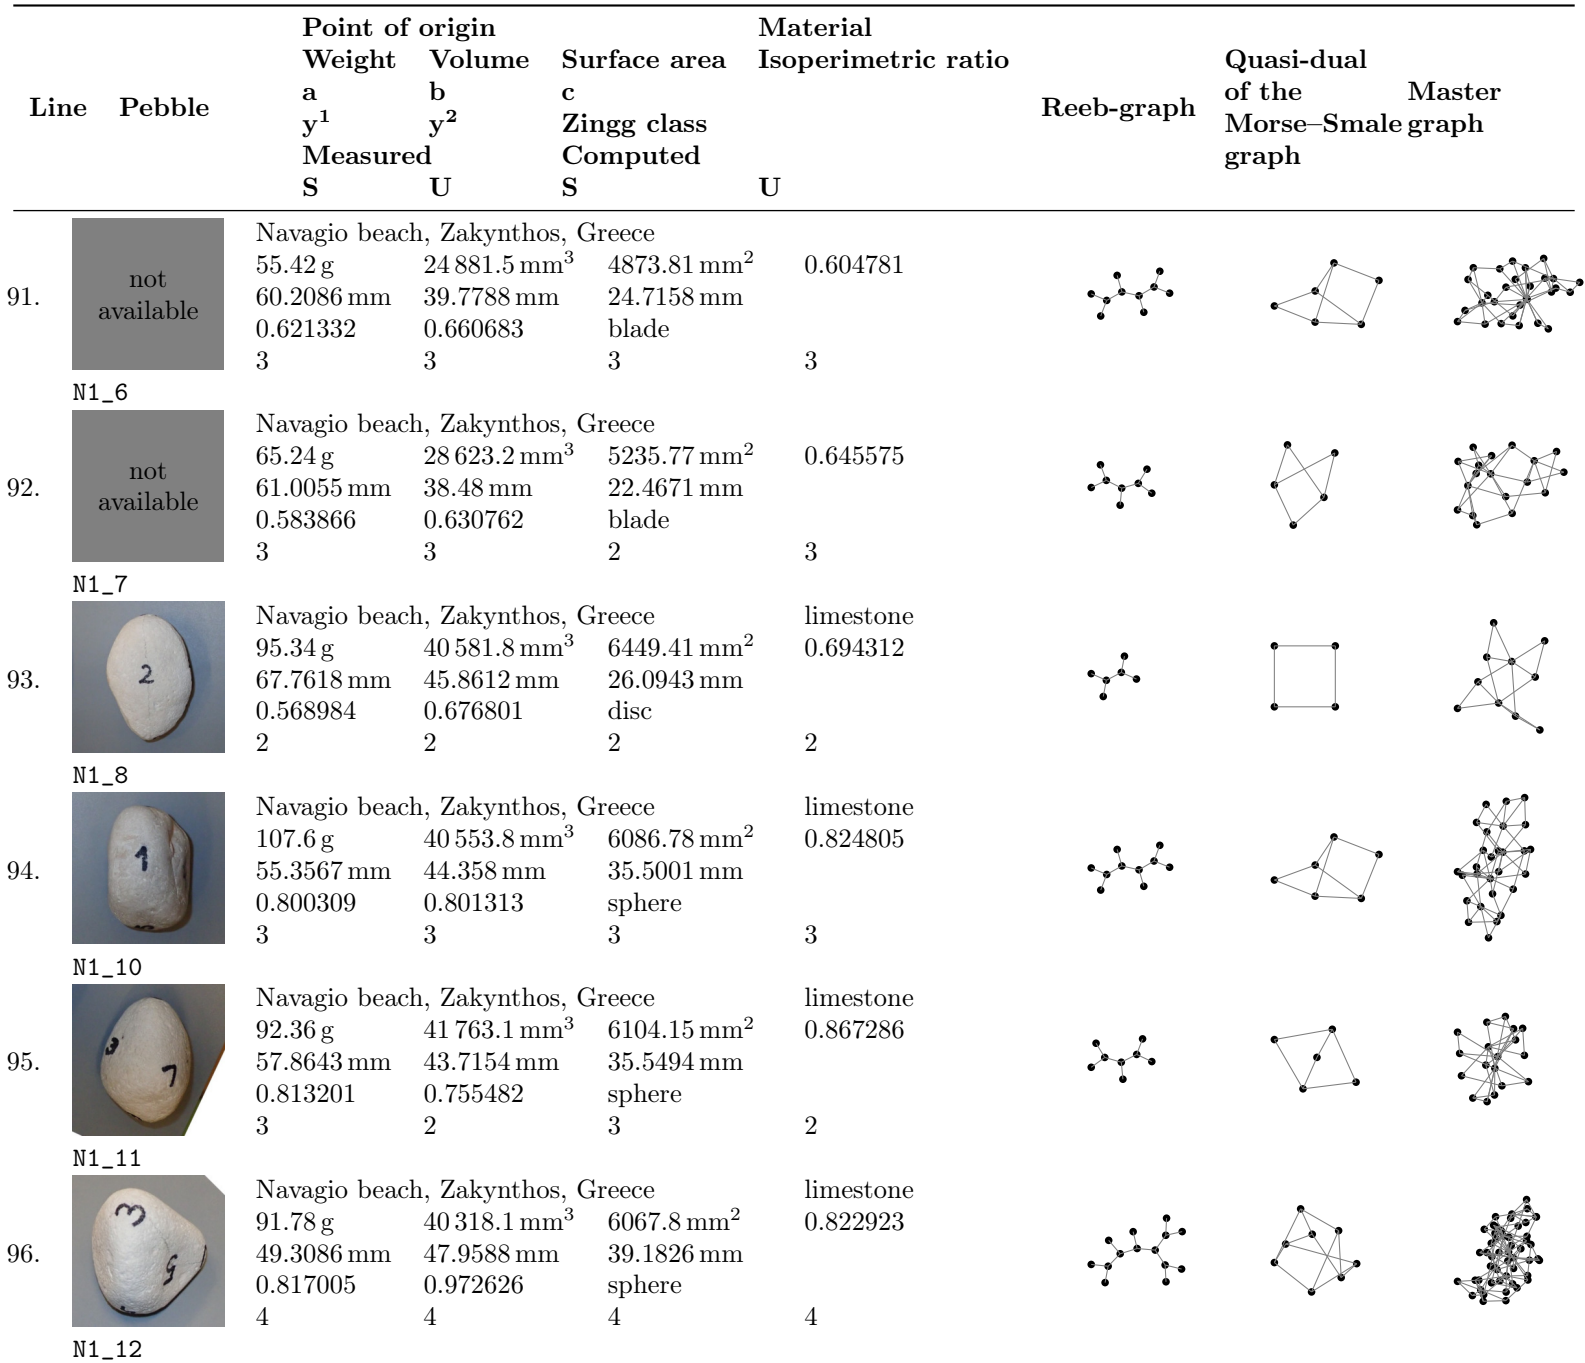 | 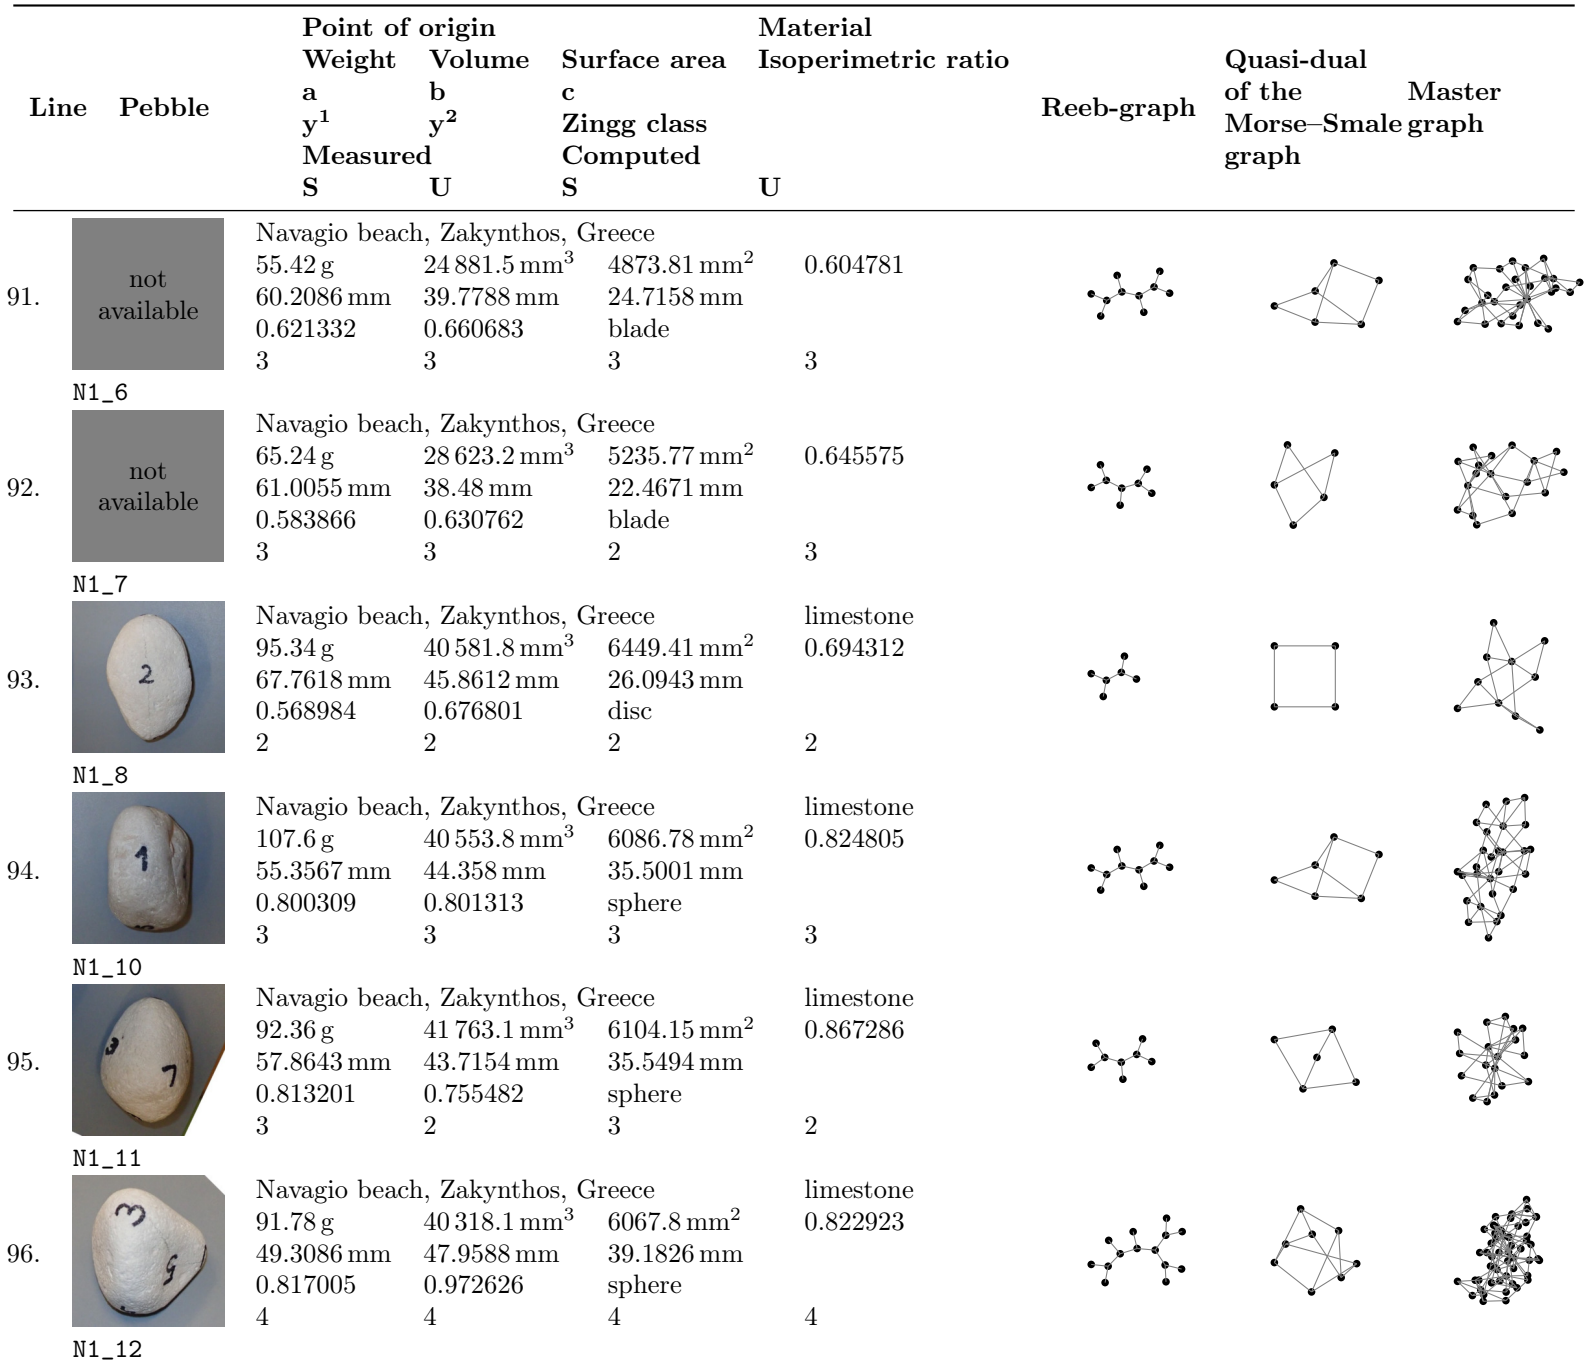 |
|      |                                                                                     | 92.36 g                              | 41 763.1 mm <sup>3</sup> | 6104.15 mm <sup>2</sup>                           |                                      |                                                                                       |                                                                                       |                                                                                       |
|      |                                                                                     | 57.8643 mm                           | 43.7154 mm               | 35.5494 mm                                        |                                      |                                                                                       |                                                                                       |                                                                                       |
|      |                                                                                     | 0.813201                             | 0.755482                 | sphere                                            |                                      |                                                                                       |                                                                                       |                                                                                       |
|      | N1_11                                                                               | 3                                    | 2                        | 3                                                 | 2                                    |                                                                                       |                                                                                       |                                                                                       |
| 96.  | 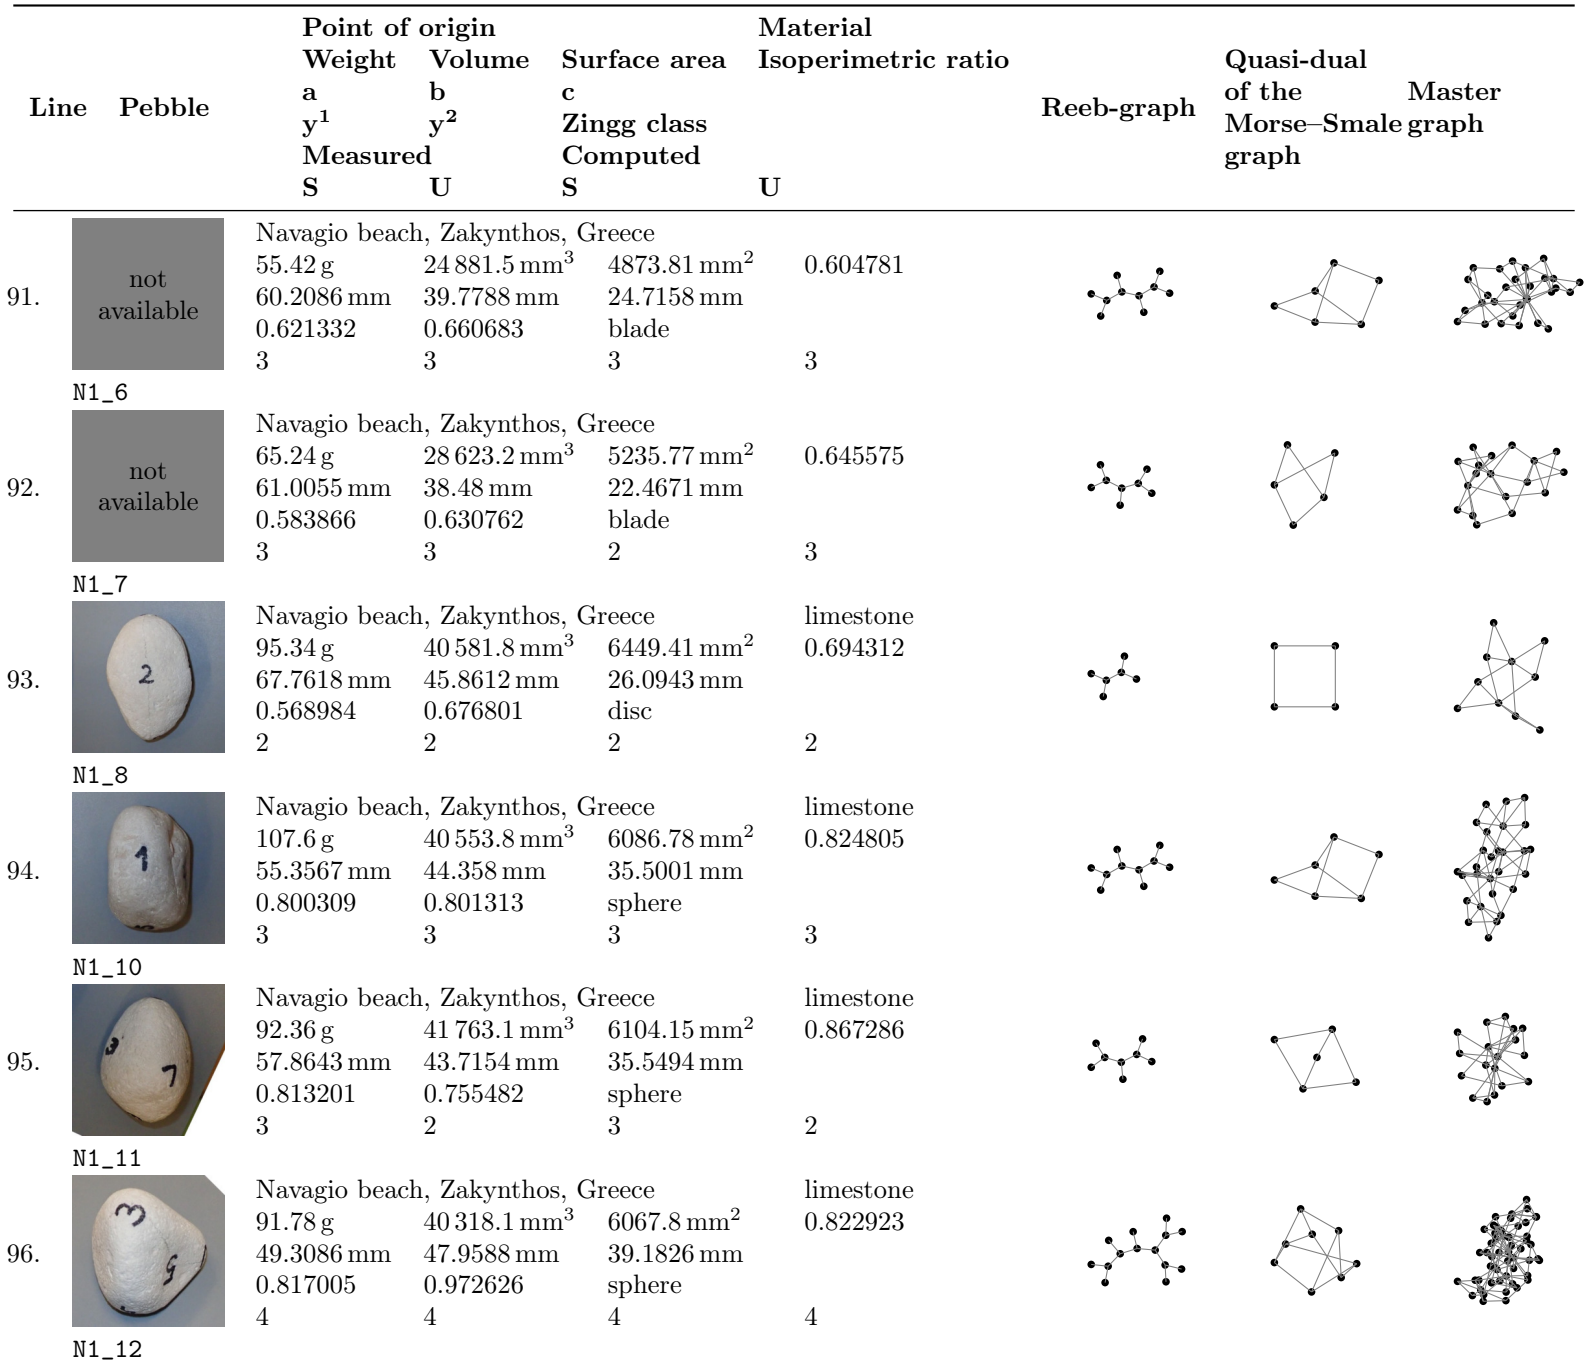 | Navagio beach, Zakynthos, Greece     |                          |                                                   | limestone<br>0.822923                | 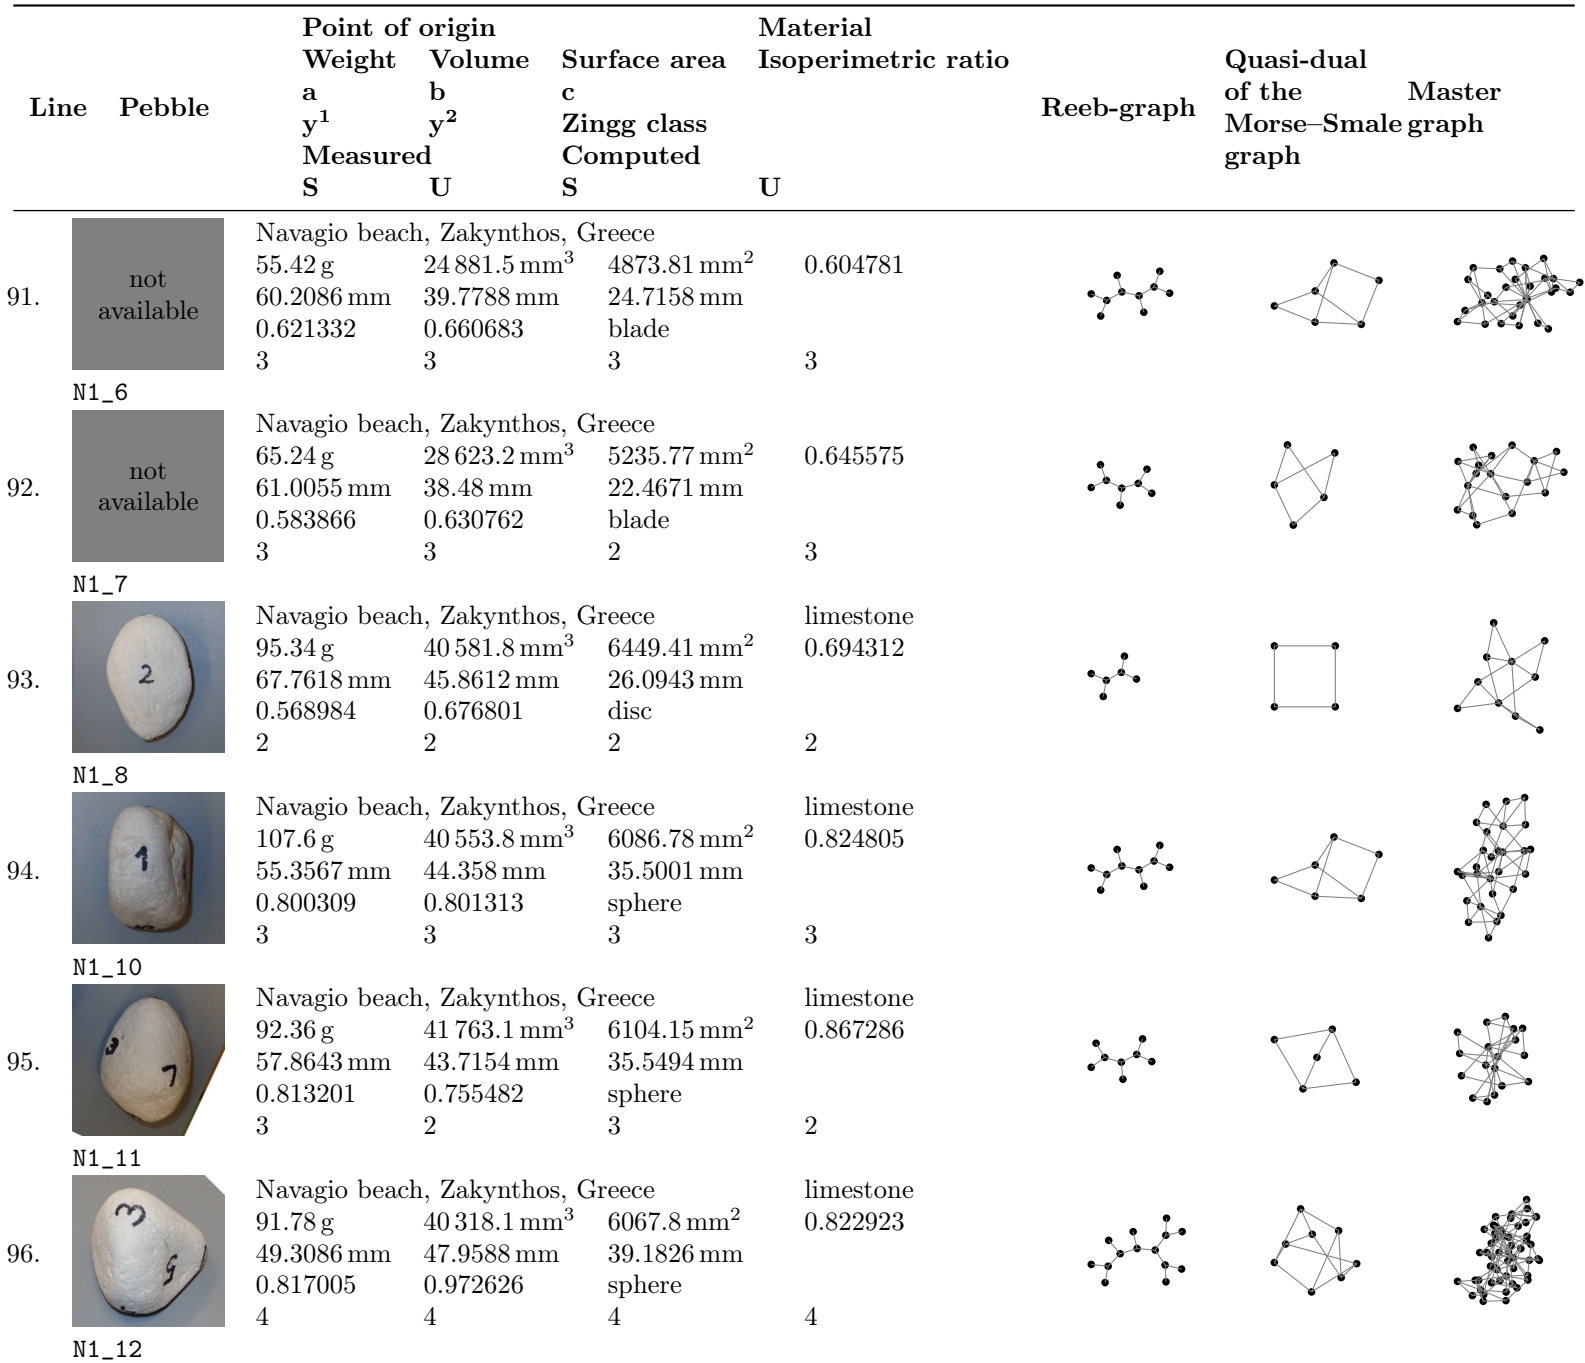 | 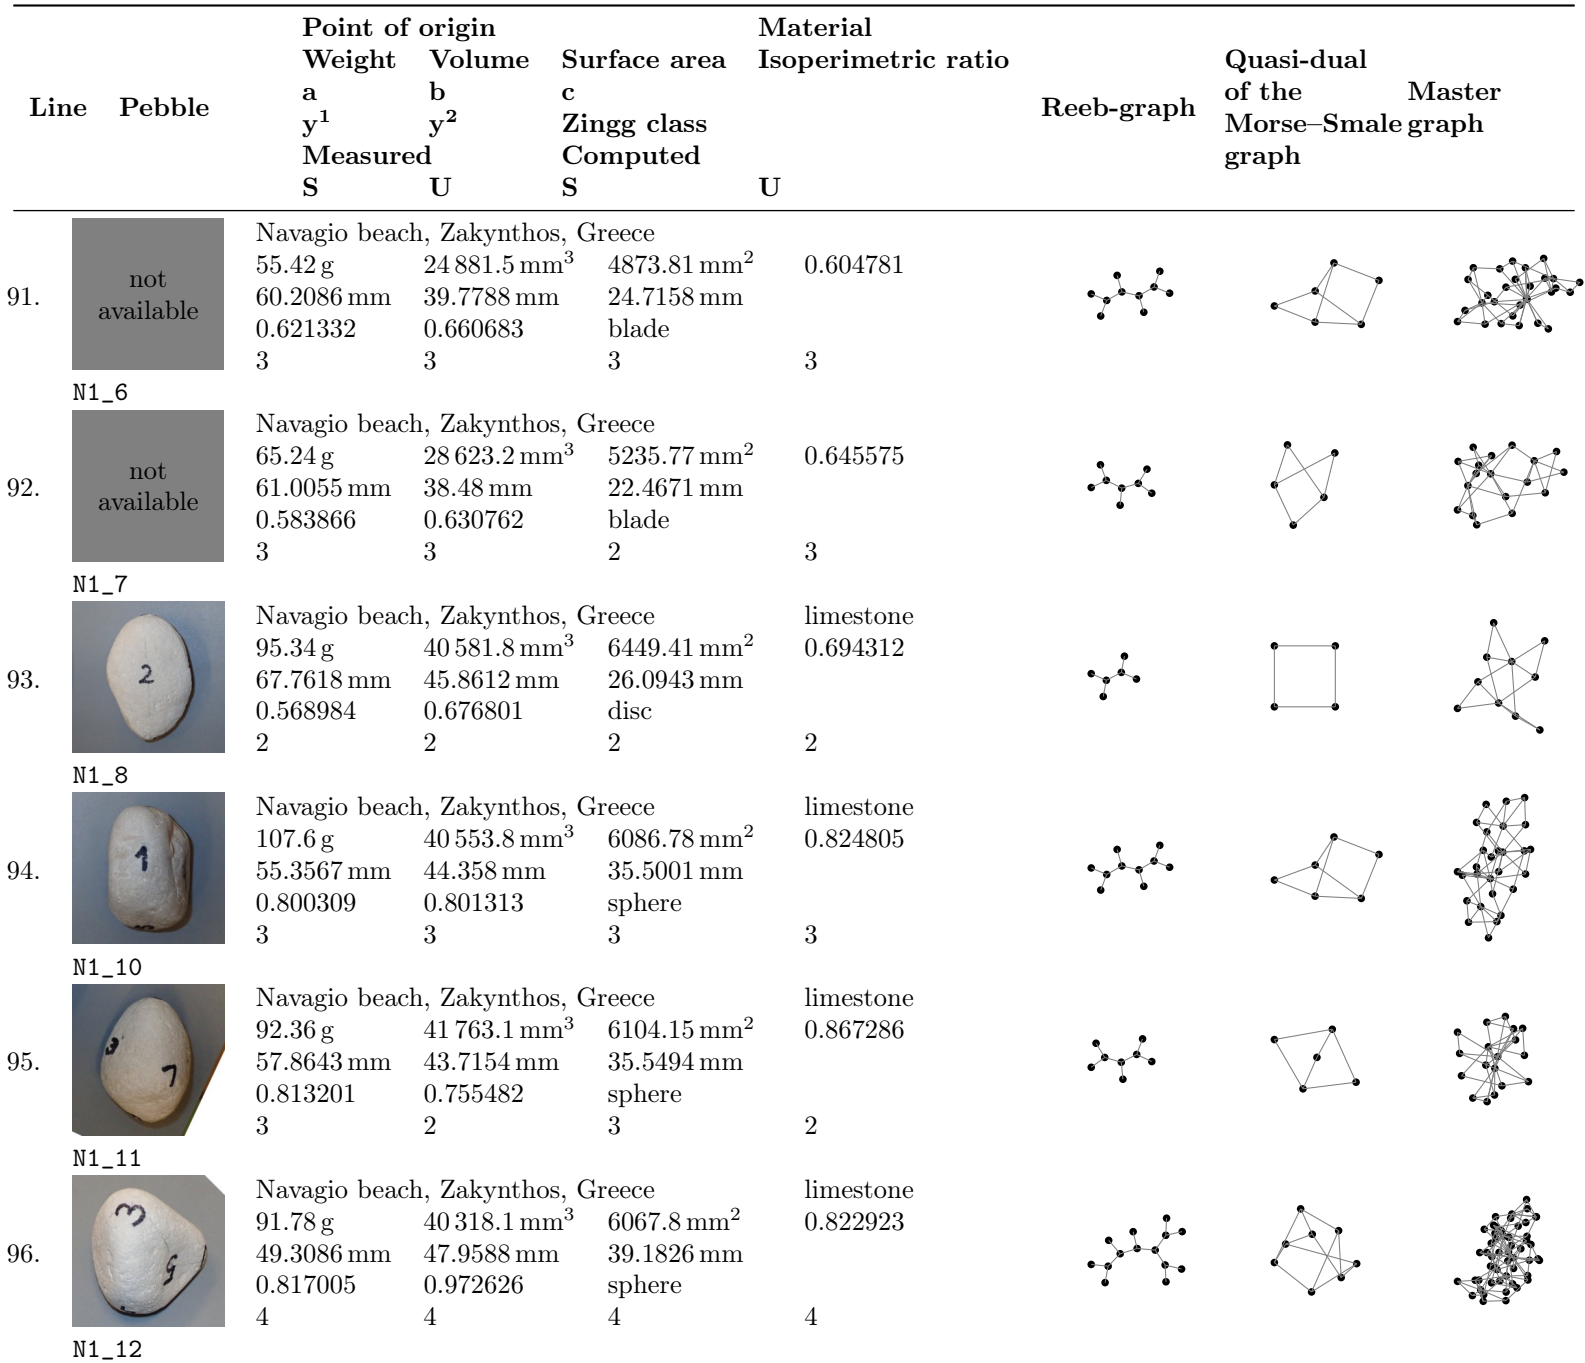 | 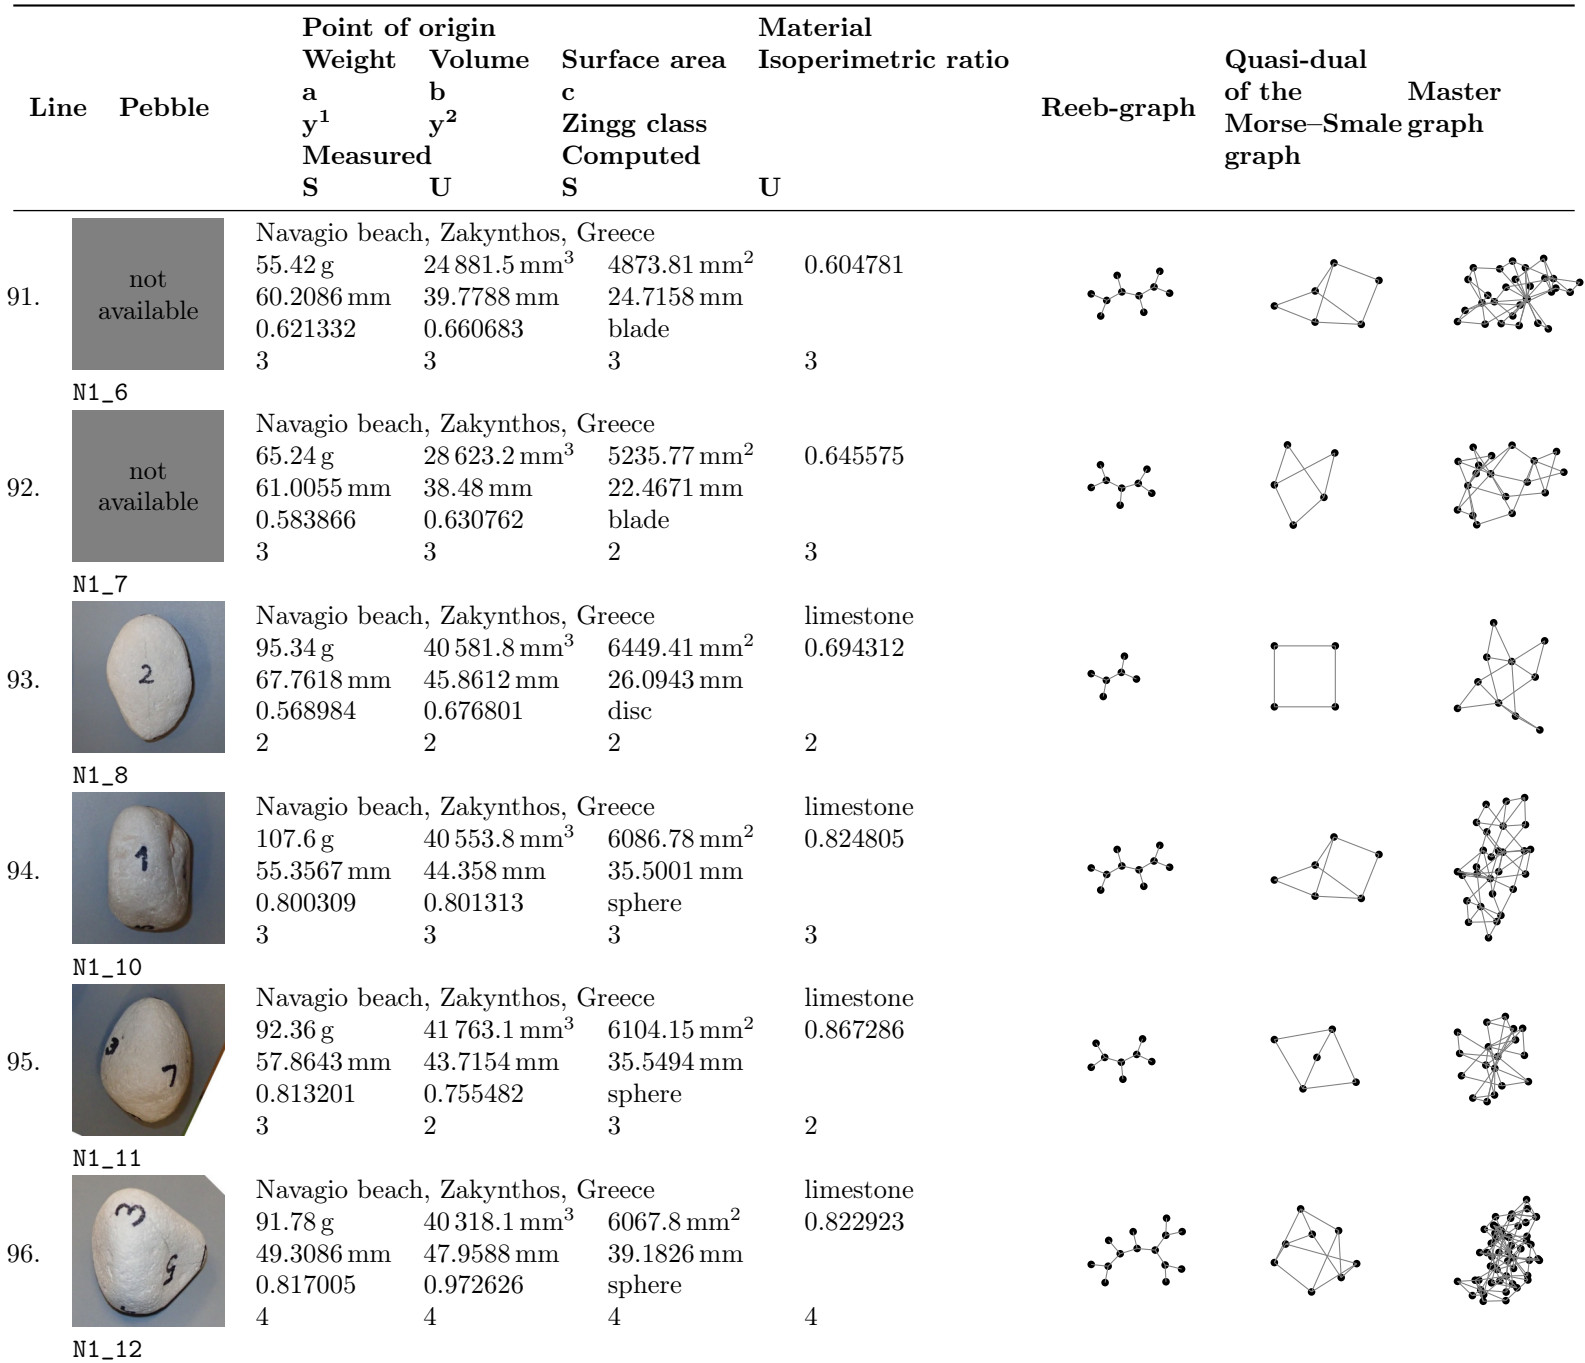 |
|      |                                                                                     | 91.78 g                              | 40 318.1 mm <sup>3</sup> | 6067.8 mm <sup>2</sup>                            |                                      |                                                                                       |                                                                                       |                                                                                       |
|      |                                                                                     | 49.3086 mm                           | 47.9588 mm               | 39.1826 mm                                        |                                      |                                                                                       |                                                                                       |                                                                                       |
|      |                                                                                     | 0.817005                             | 0.972626                 | sphere                                            |                                      |                                                                                       |                                                                                       |                                                                                       |
|      | N1_12                                                                               | 4                                    | 4                        | 4                                                 | 4                                    |                                                                                       |                                                                                       |                                                                                       |

| Line | Pebble                                                                              | Point of origin                                                             |                                                         |                                                      | Material              | Reeb-graph                                                                            | Quasi-dual<br>of the<br>Morse–Smale<br>graph                                          | Master<br>graph                                                                       |
|------|-------------------------------------------------------------------------------------|-----------------------------------------------------------------------------|---------------------------------------------------------|------------------------------------------------------|-----------------------|---------------------------------------------------------------------------------------|---------------------------------------------------------------------------------------|---------------------------------------------------------------------------------------|
|      |                                                                                     | Weight                                                                      | Volume                                                  | Surface area                                         |                       |                                                                                       |                                                                                       |                                                                                       |
|      |                                                                                     | a                                                                           | b                                                       | c                                                    |                       |                                                                                       |                                                                                       |                                                                                       |
|      |                                                                                     | y <sup>1</sup><br>Measured<br>S                                             | y <sup>2</sup><br>U                                     | Zingg class<br>Computed<br>S                         |                       |                                                                                       |                                                                                       |                                                                                       |
| 97.  | 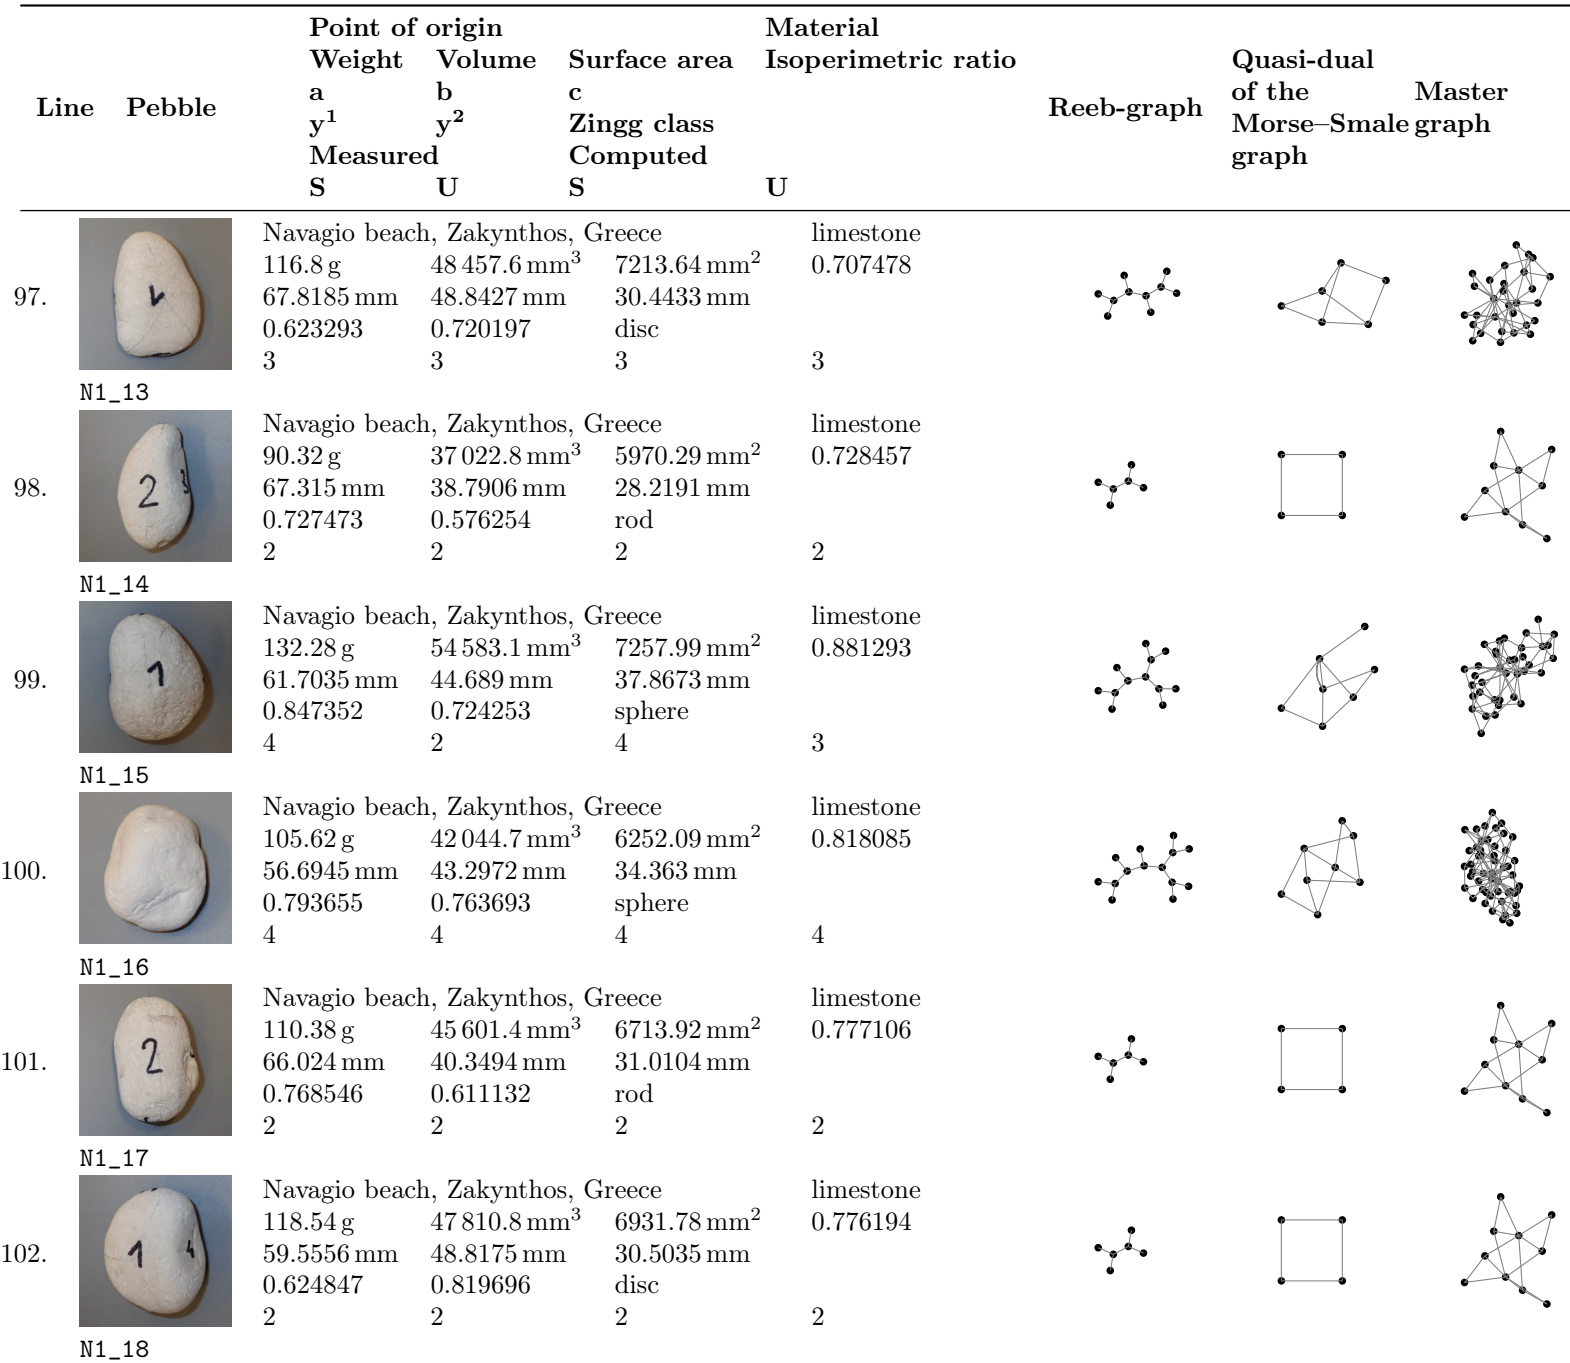   | Navagio beach, Zakynthos, Greece<br>116.8 g<br>67.8185 mm<br>0.623293<br>3  | 48 457.6 mm <sup>3</sup><br>48.8427 mm<br>0.720197<br>3 | 7213.64 mm <sup>2</sup><br>30.4433 mm<br>disc<br>3   | limestone<br>0.707478 | 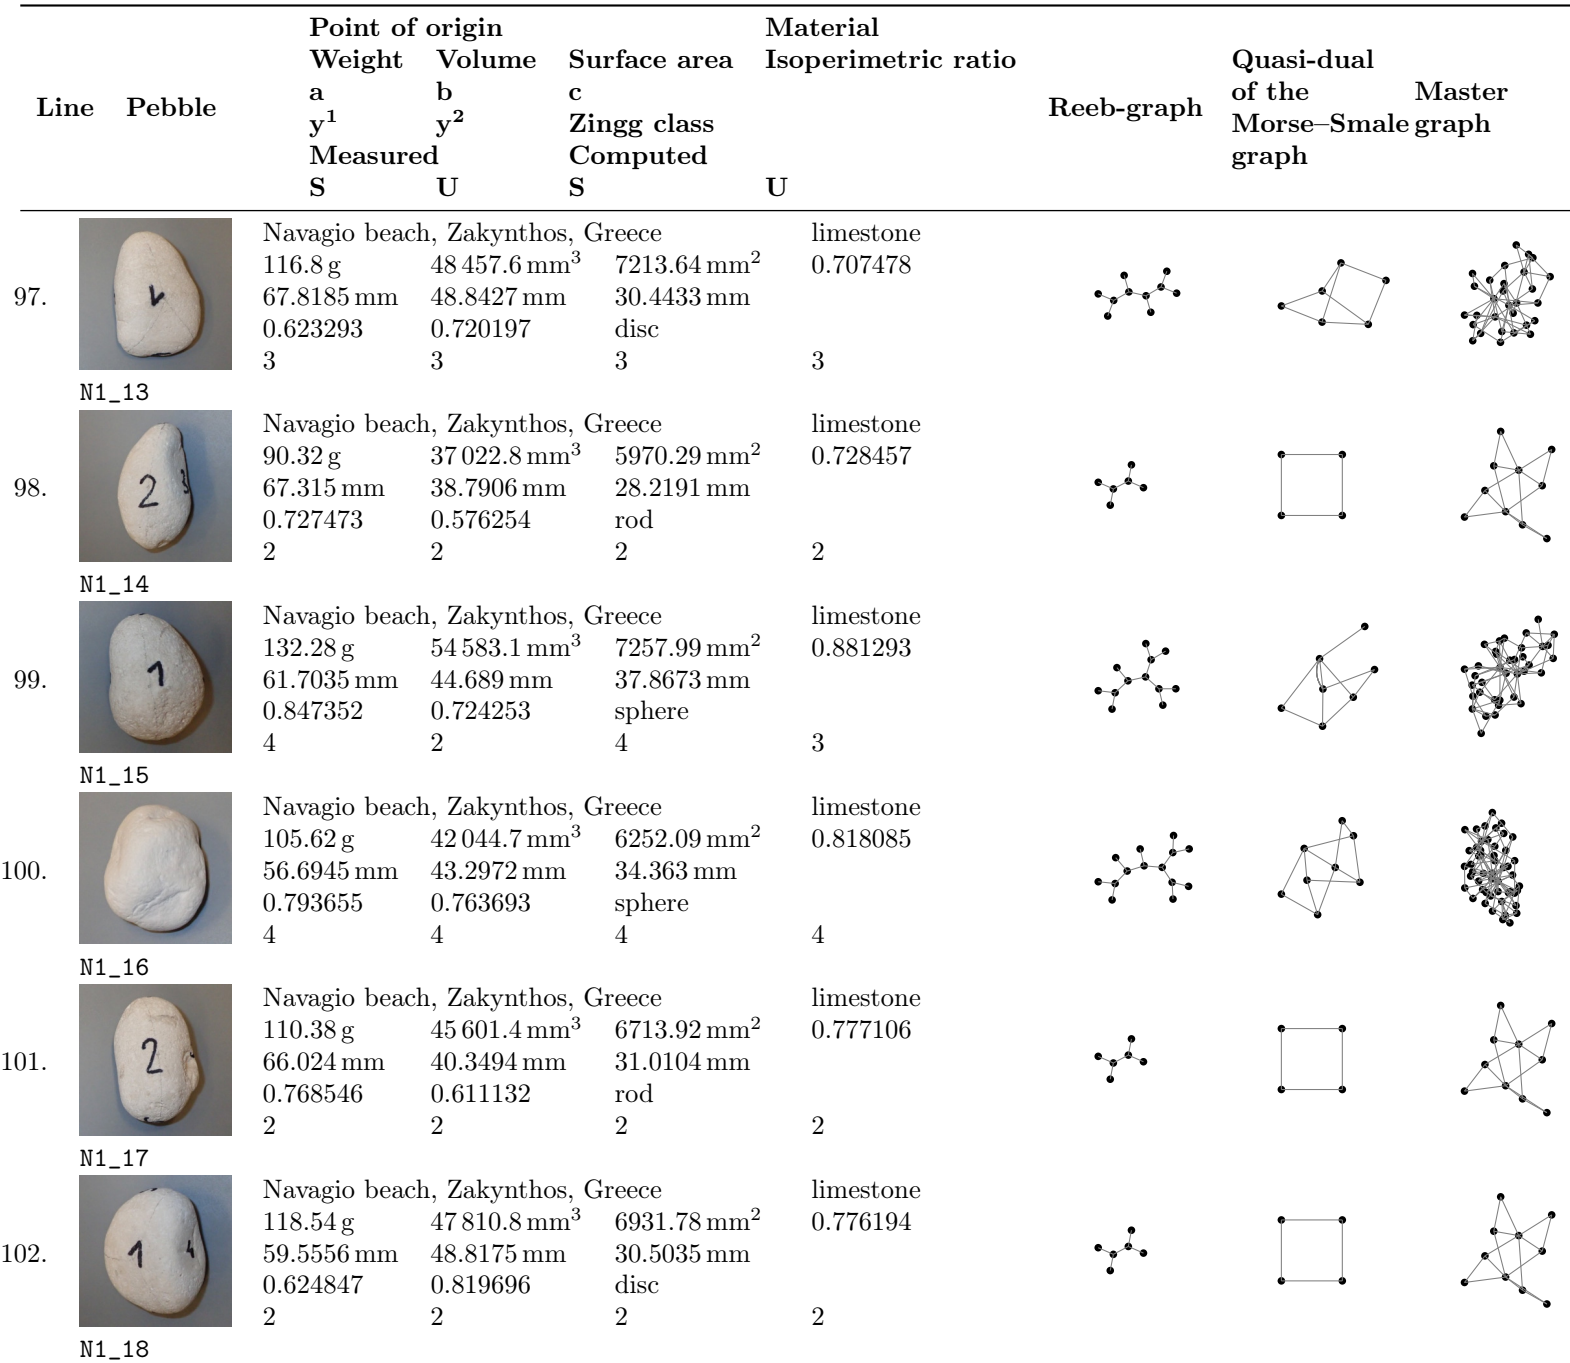   | 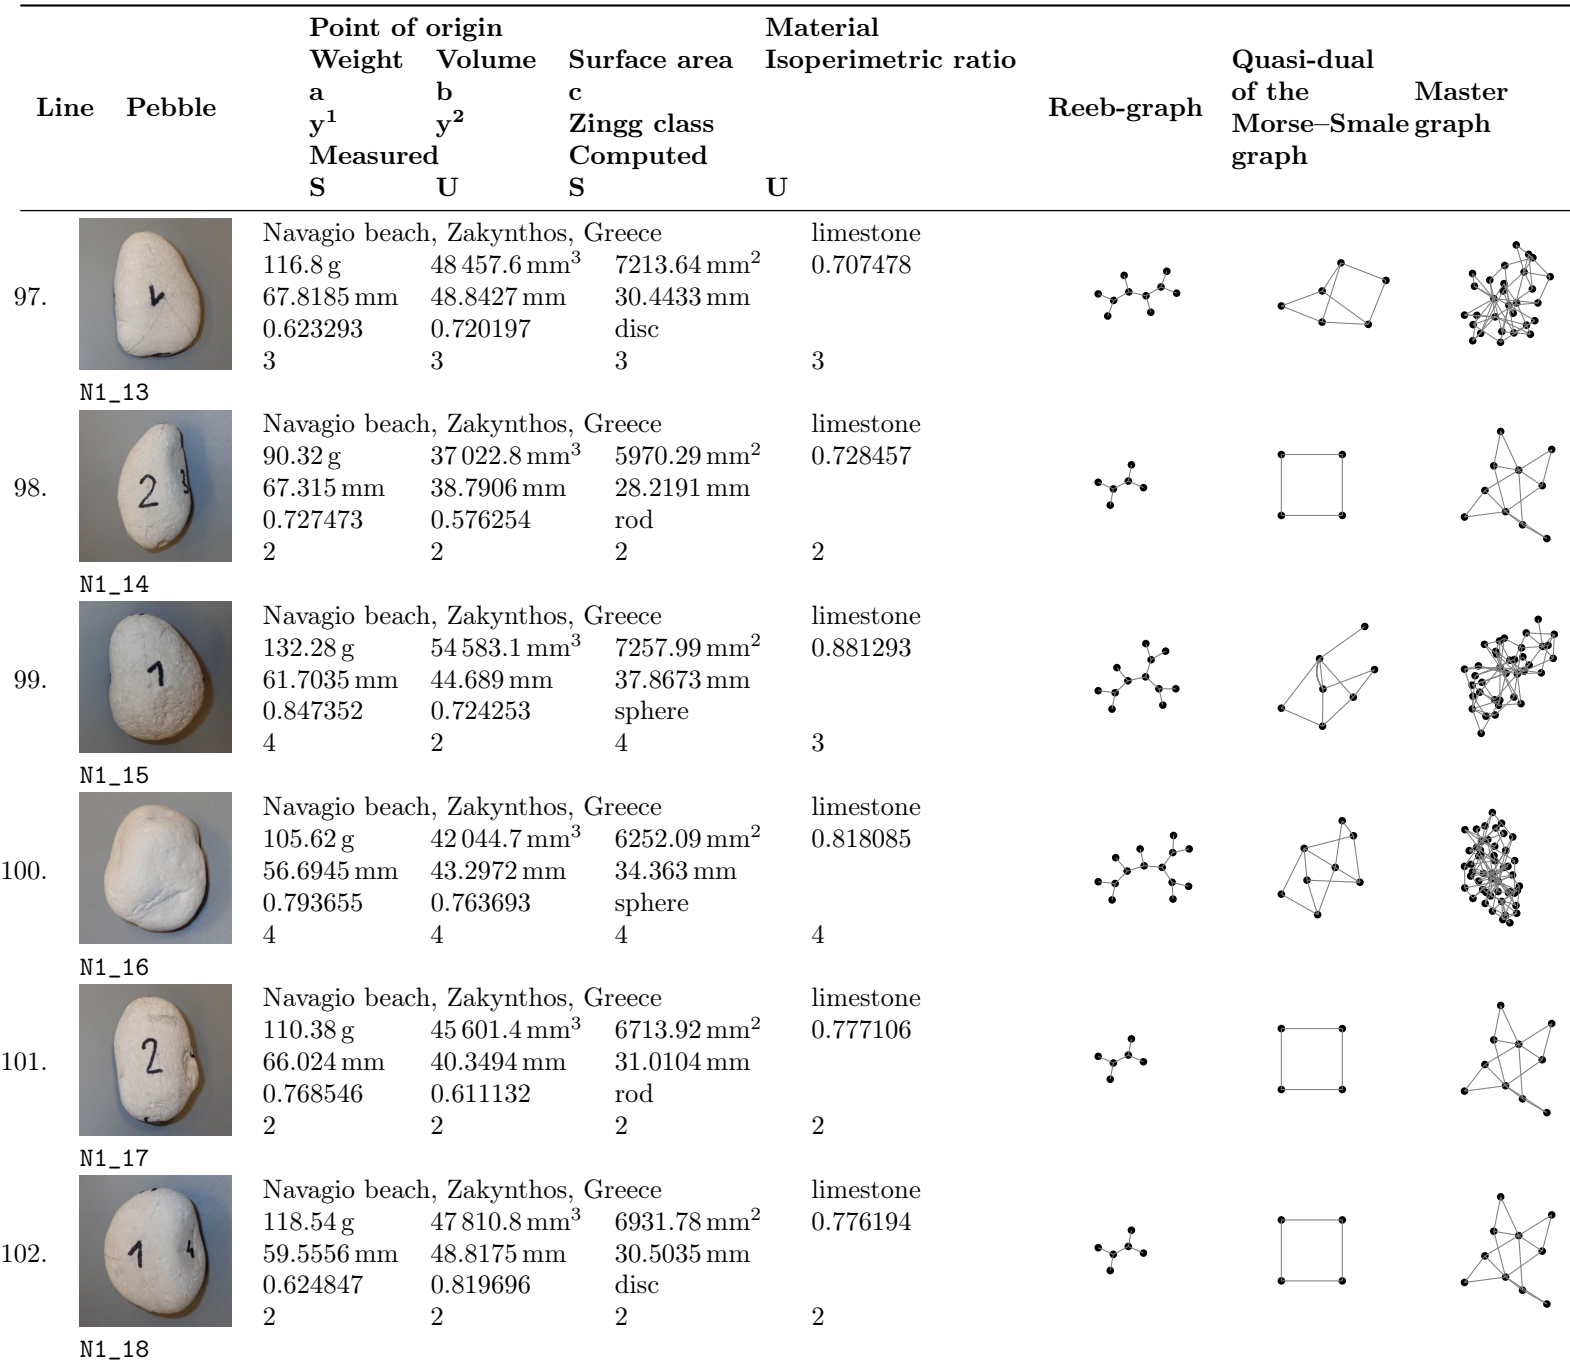   | 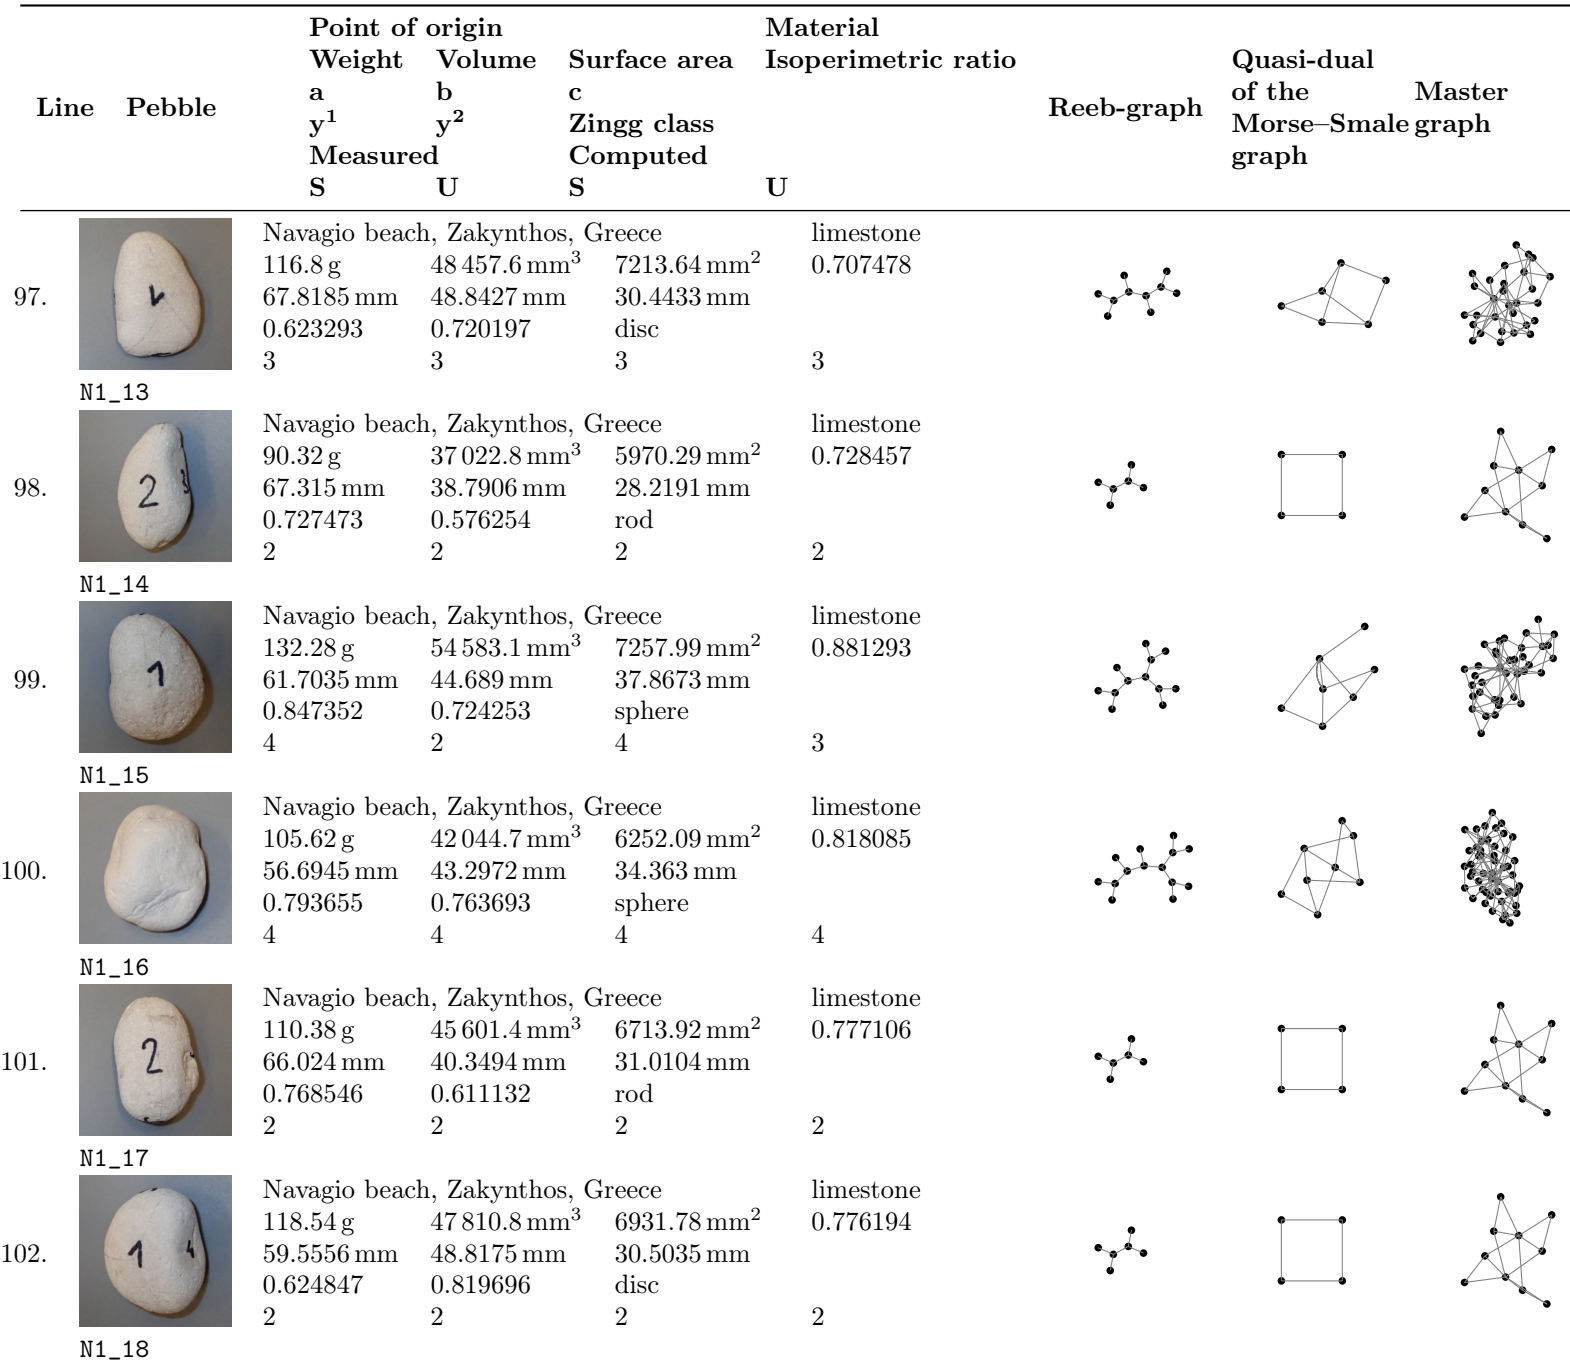   |
|      | N1_13                                                                               |                                                                             |                                                         |                                                      |                       |                                                                                       |                                                                                       |                                                                                       |
| 98.  | 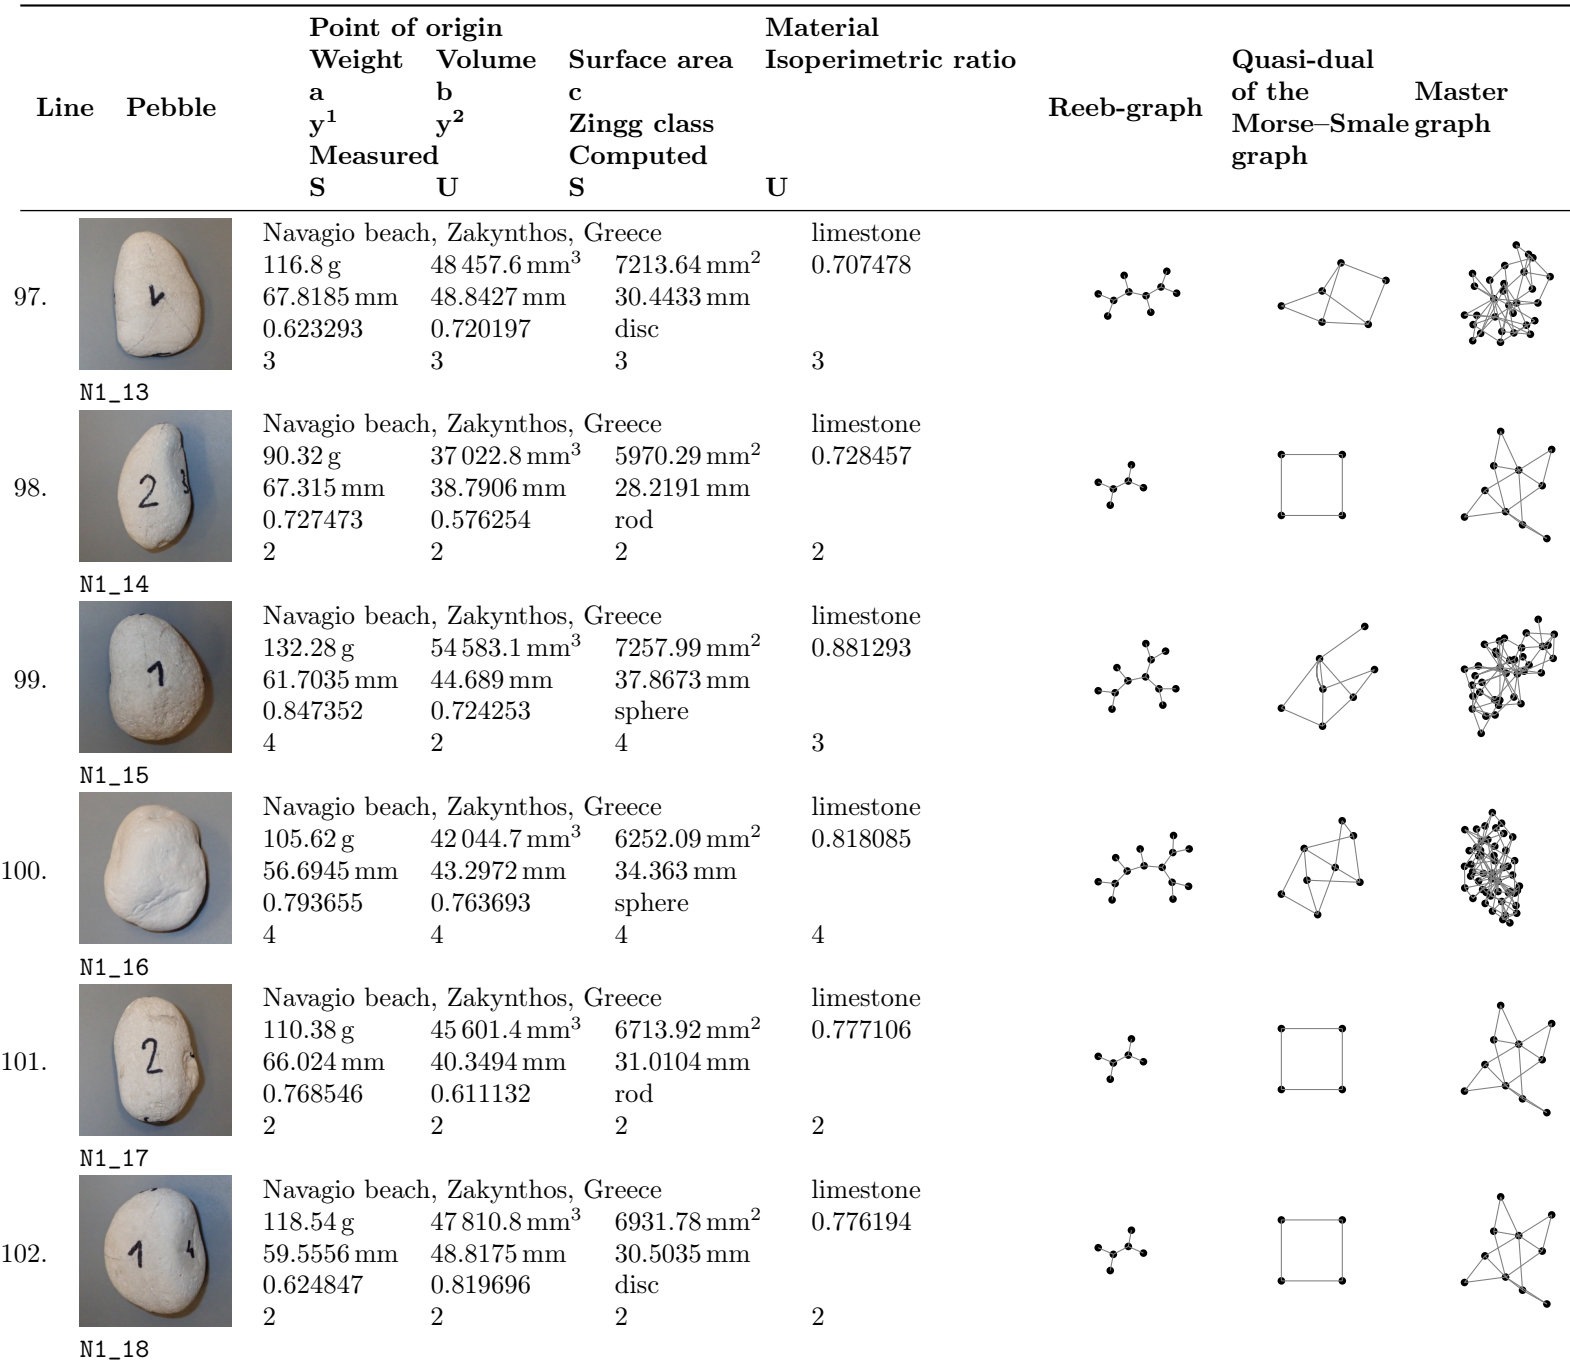   | Navagio beach, Zakynthos, Greece<br>90.32 g<br>67.315 mm<br>0.727473<br>2   | 37 022.8 mm <sup>3</sup><br>38.7906 mm<br>0.576254<br>2 | 5970.29 mm <sup>2</sup><br>28.2191 mm<br>rod<br>2    | limestone<br>0.728457 | 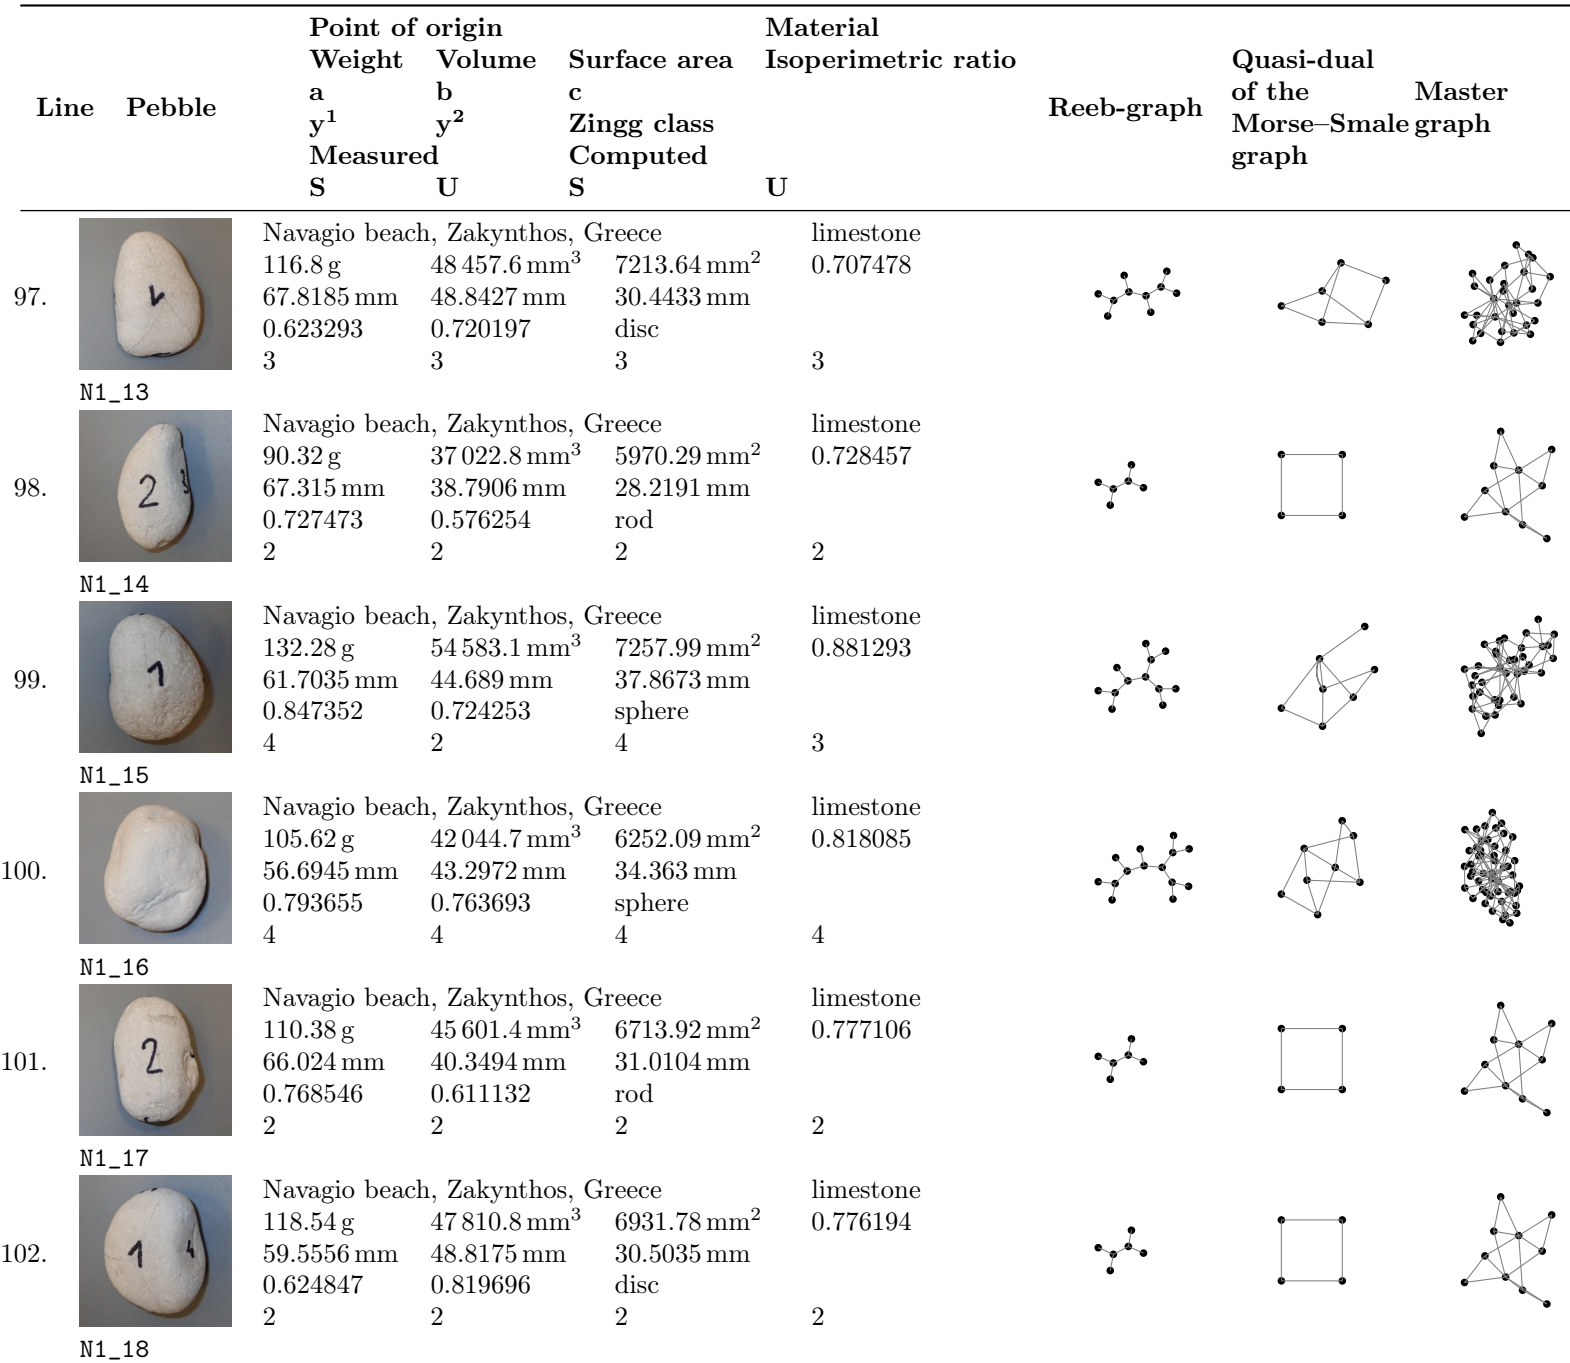   | 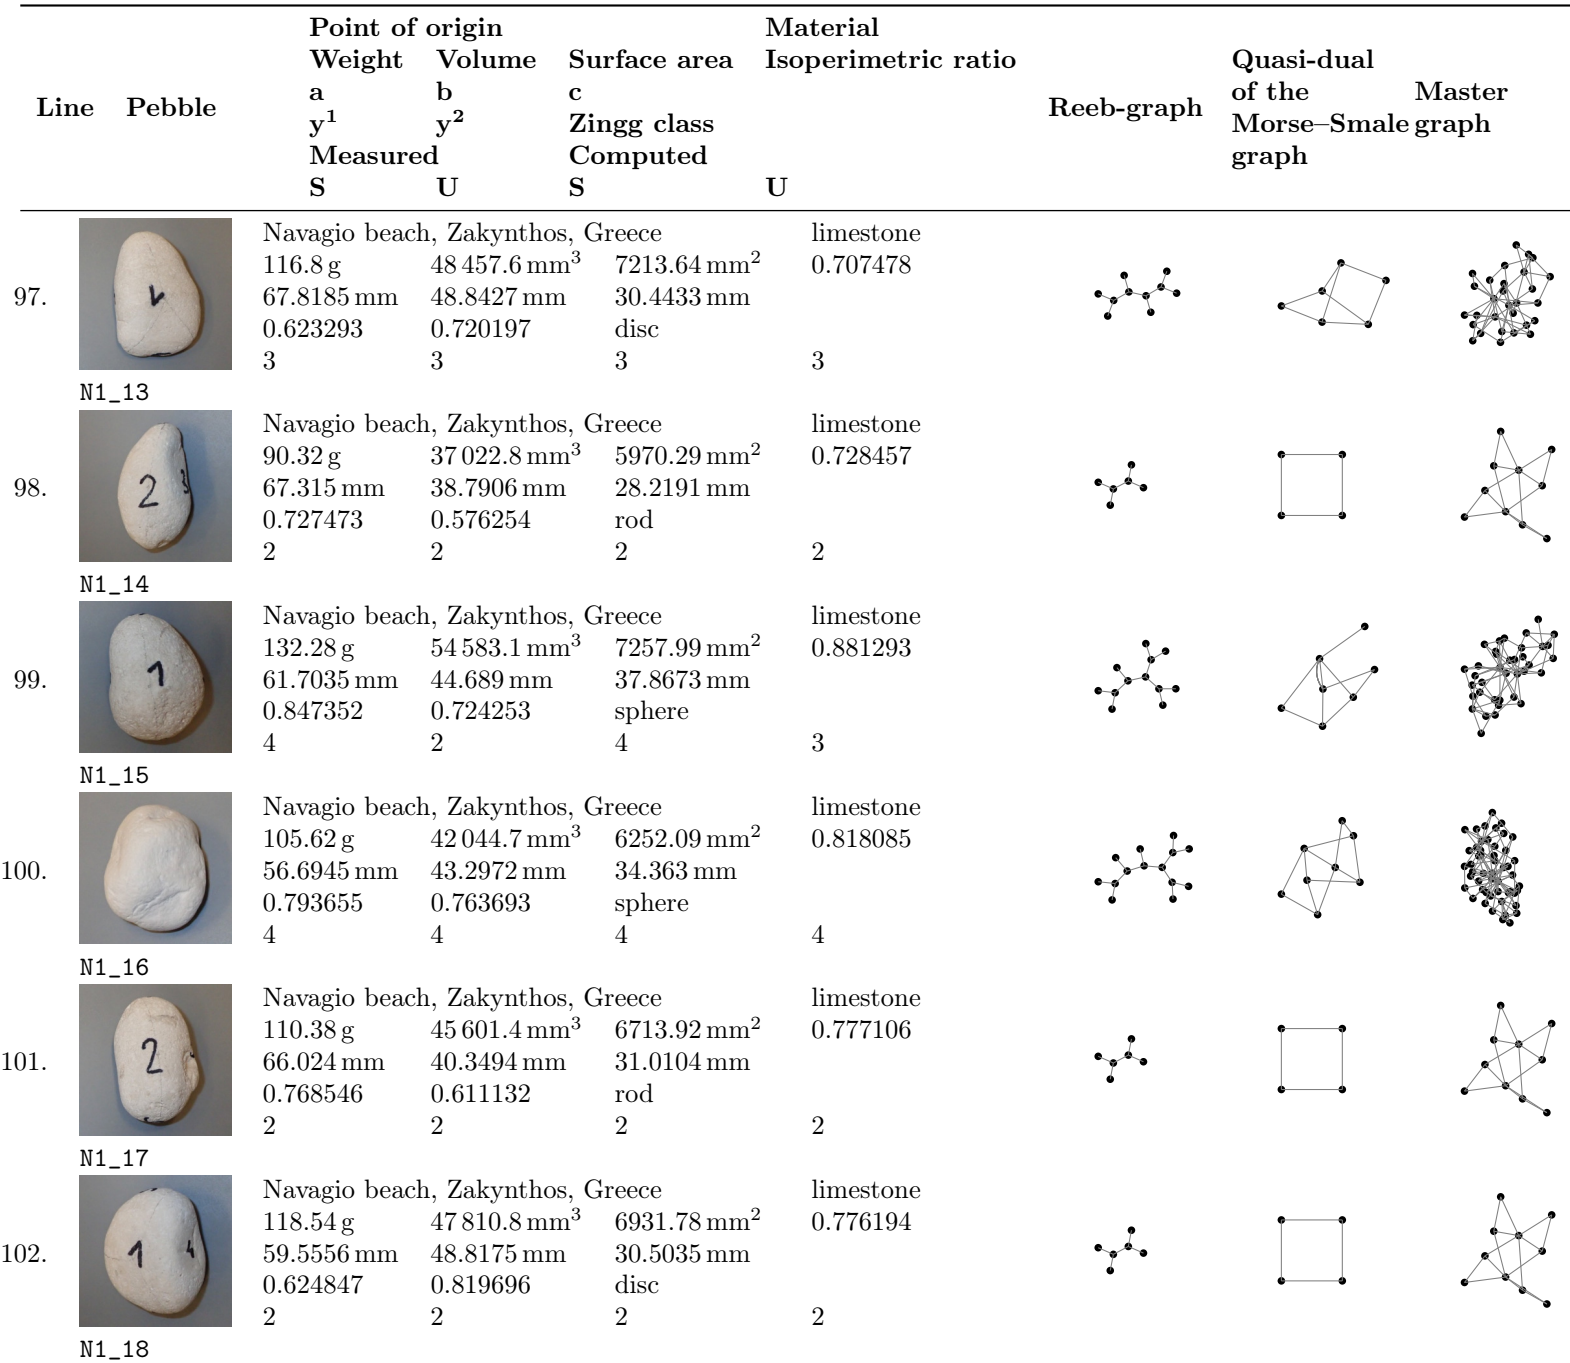   | 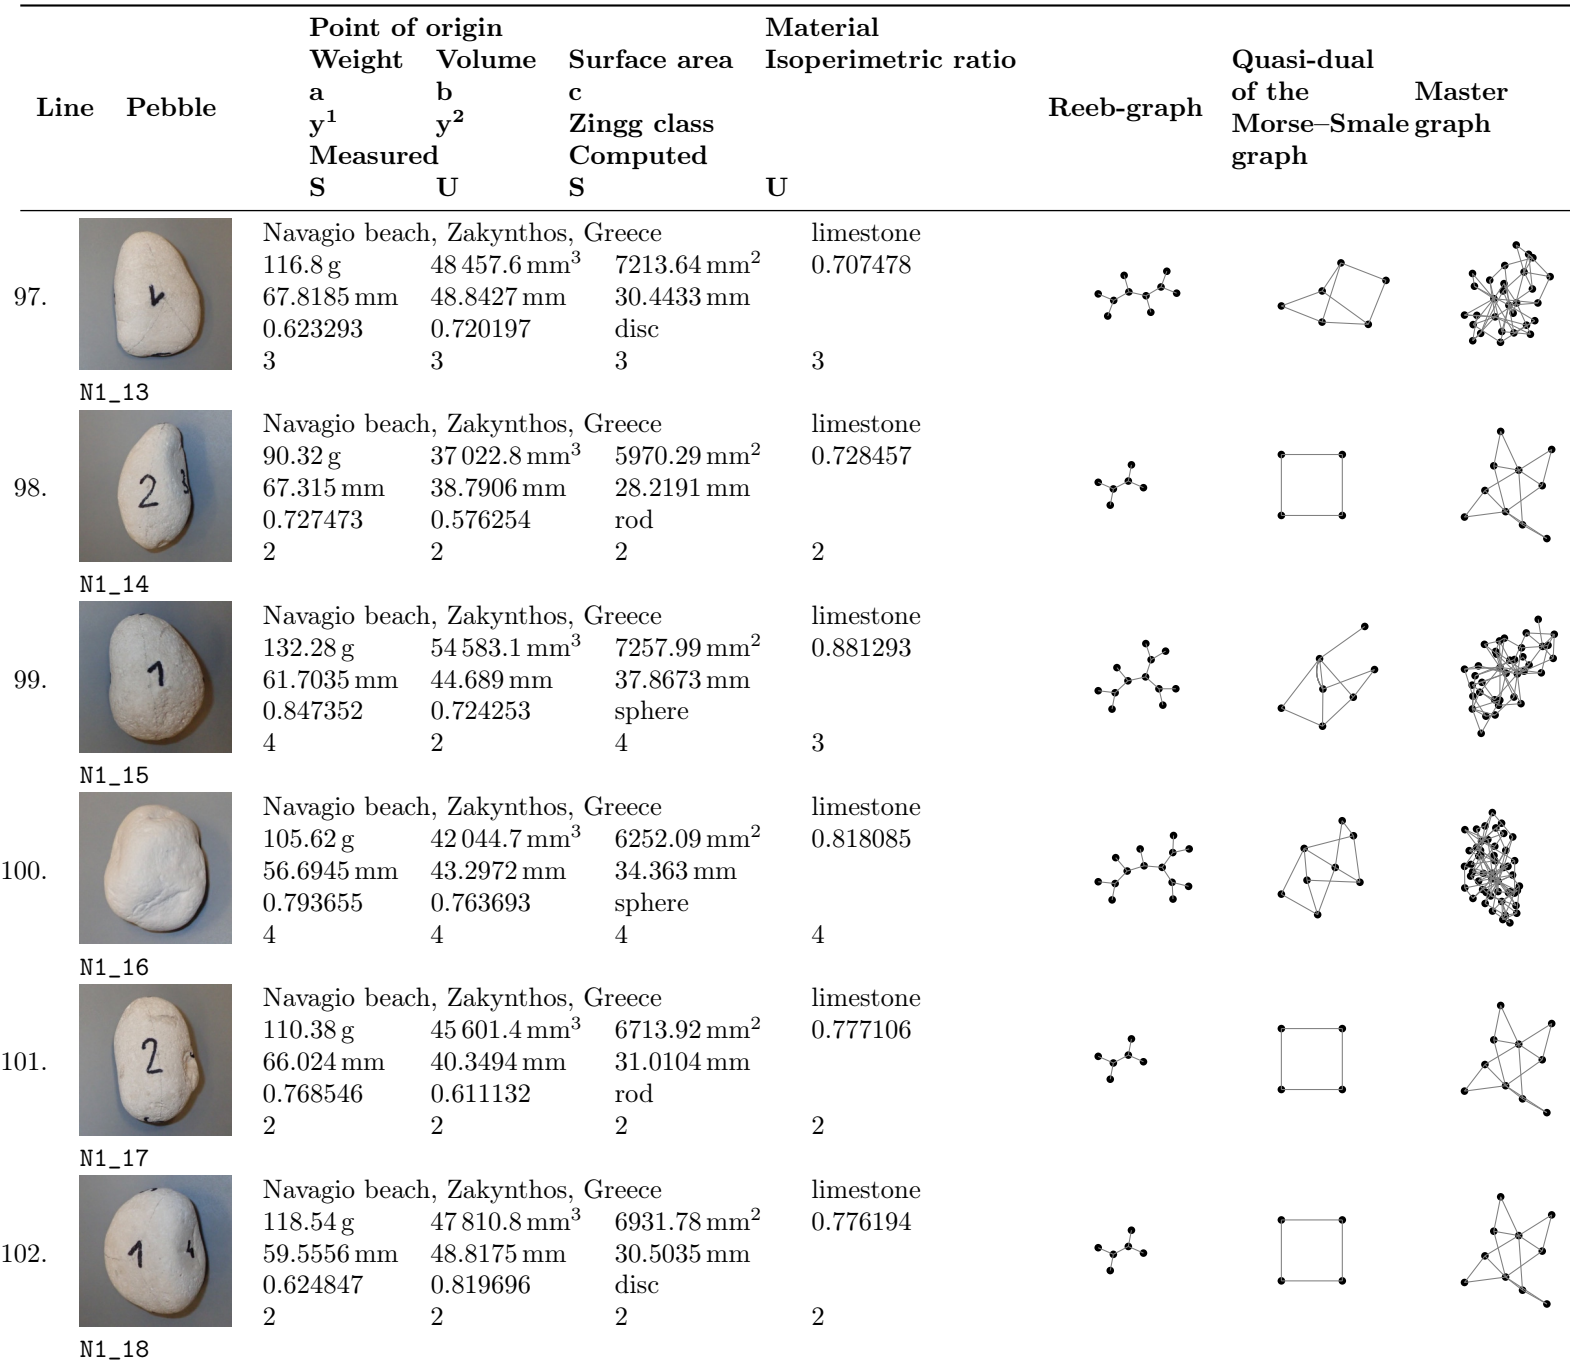   |
|      | N1_14                                                                               |                                                                             |                                                         |                                                      |                       |                                                                                       |                                                                                       |                                                                                       |
| 99.  | 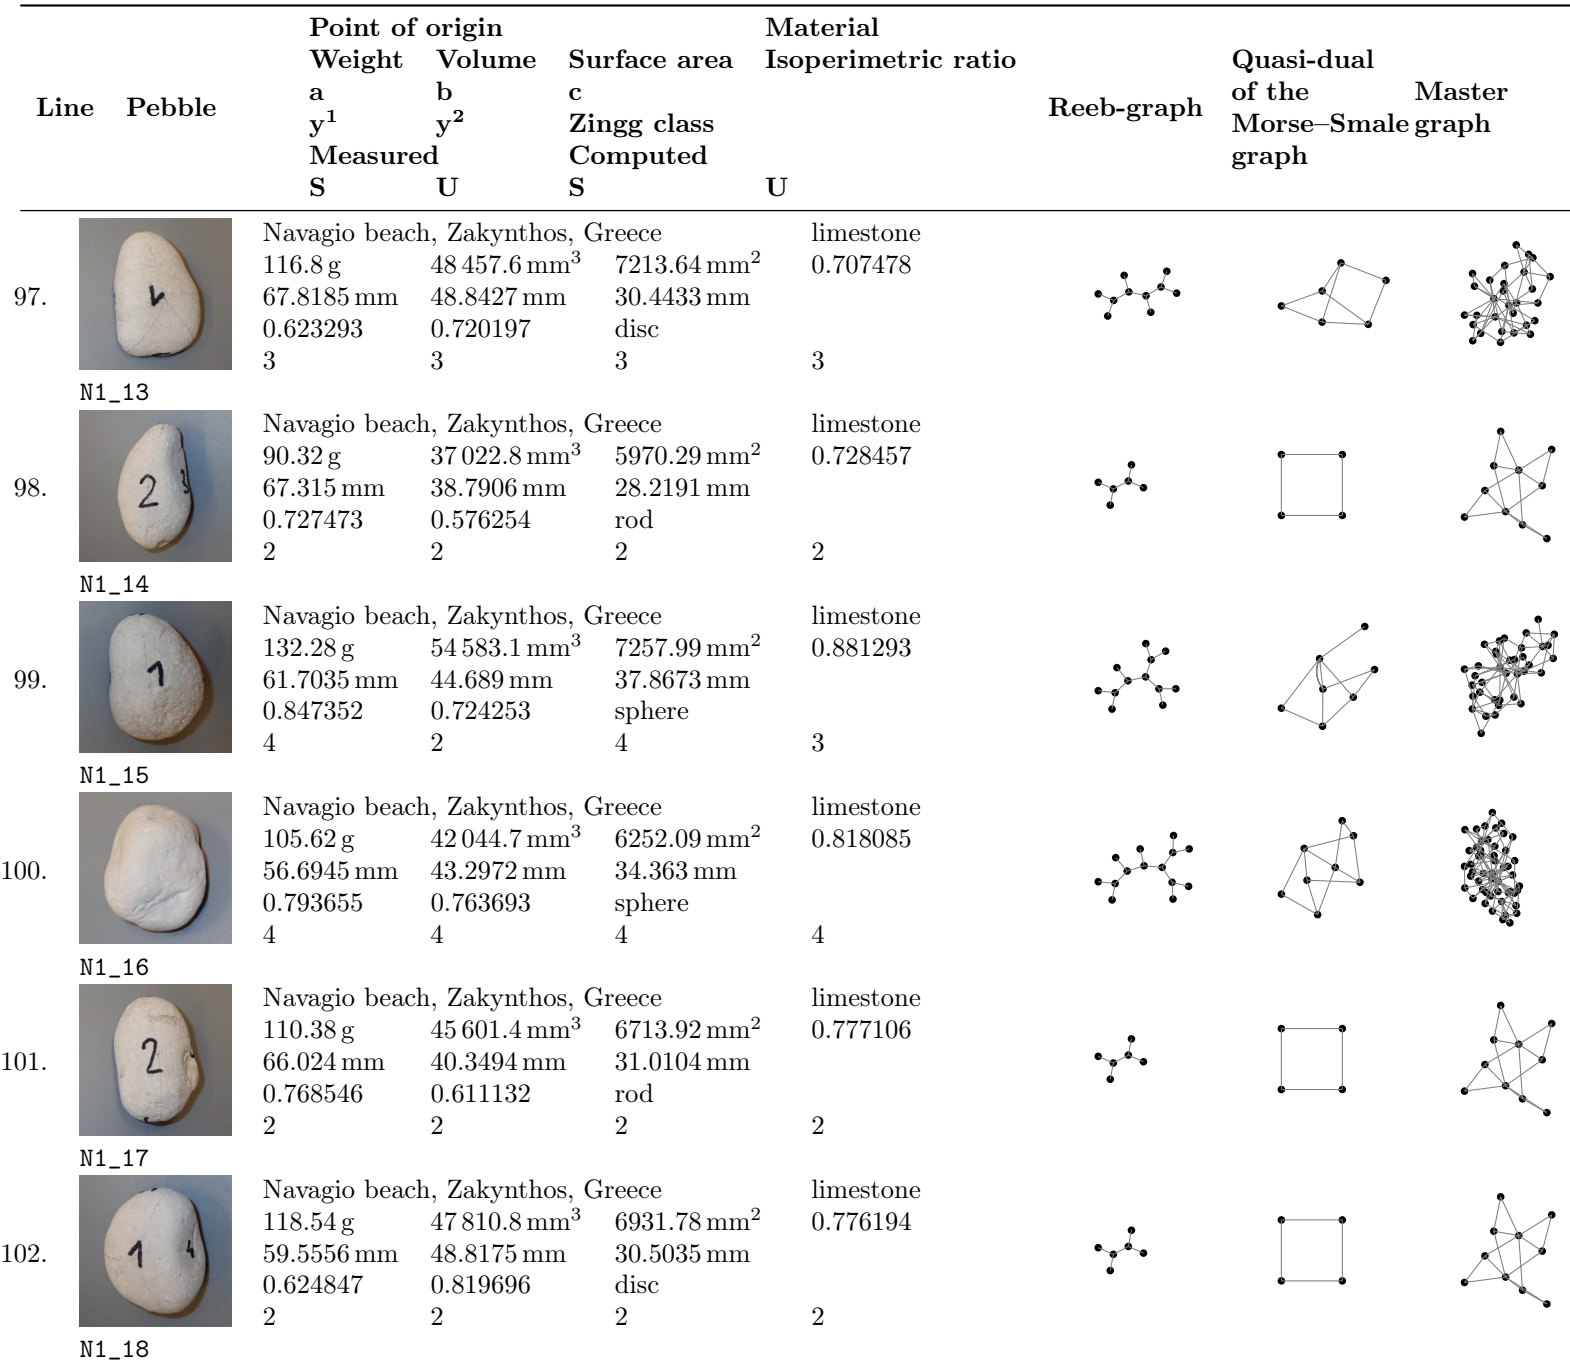   | Navagio beach, Zakynthos, Greece<br>132.28 g<br>61.7035 mm<br>0.847352<br>4 | 54 583.1 mm <sup>3</sup><br>44.689 mm<br>0.724253<br>2  | 7257.99 mm <sup>2</sup><br>37.8673 mm<br>sphere<br>4 | limestone<br>0.881293 | 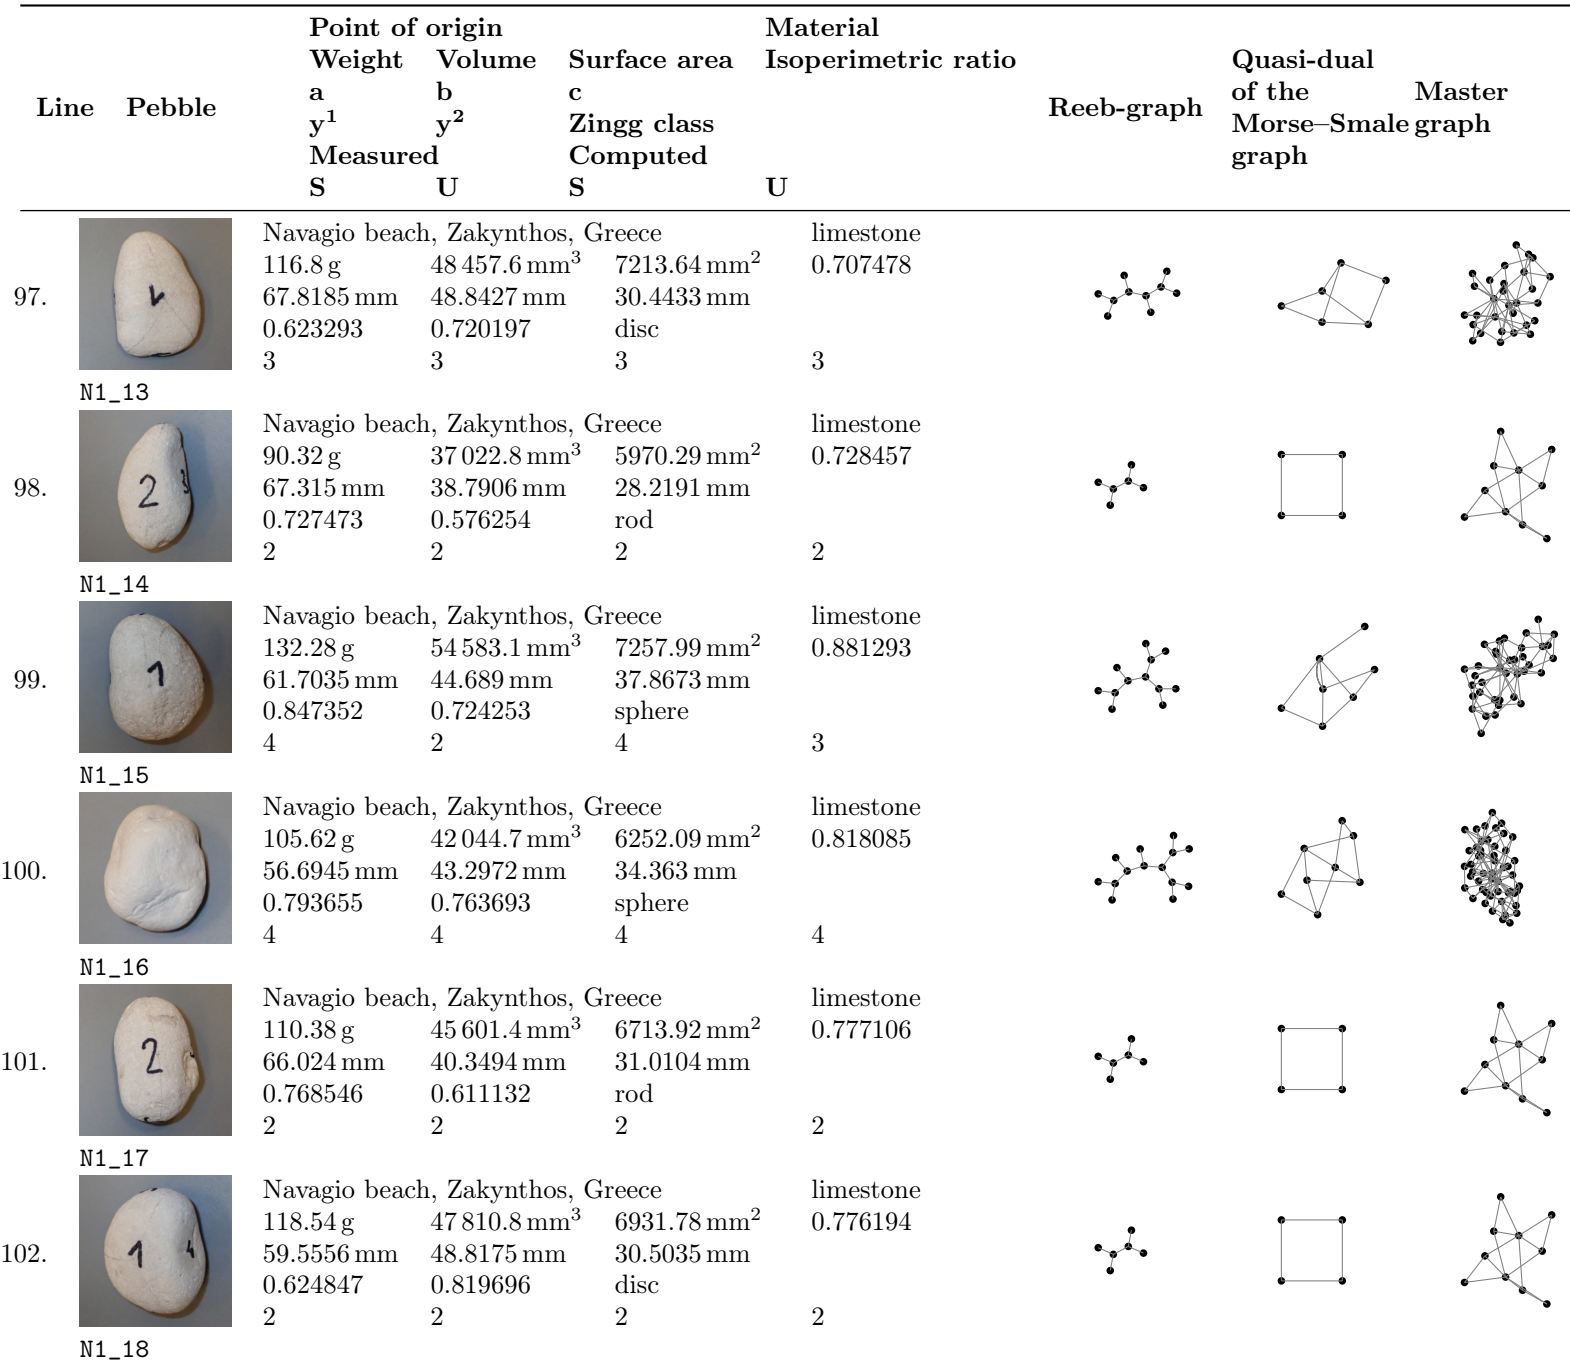   | 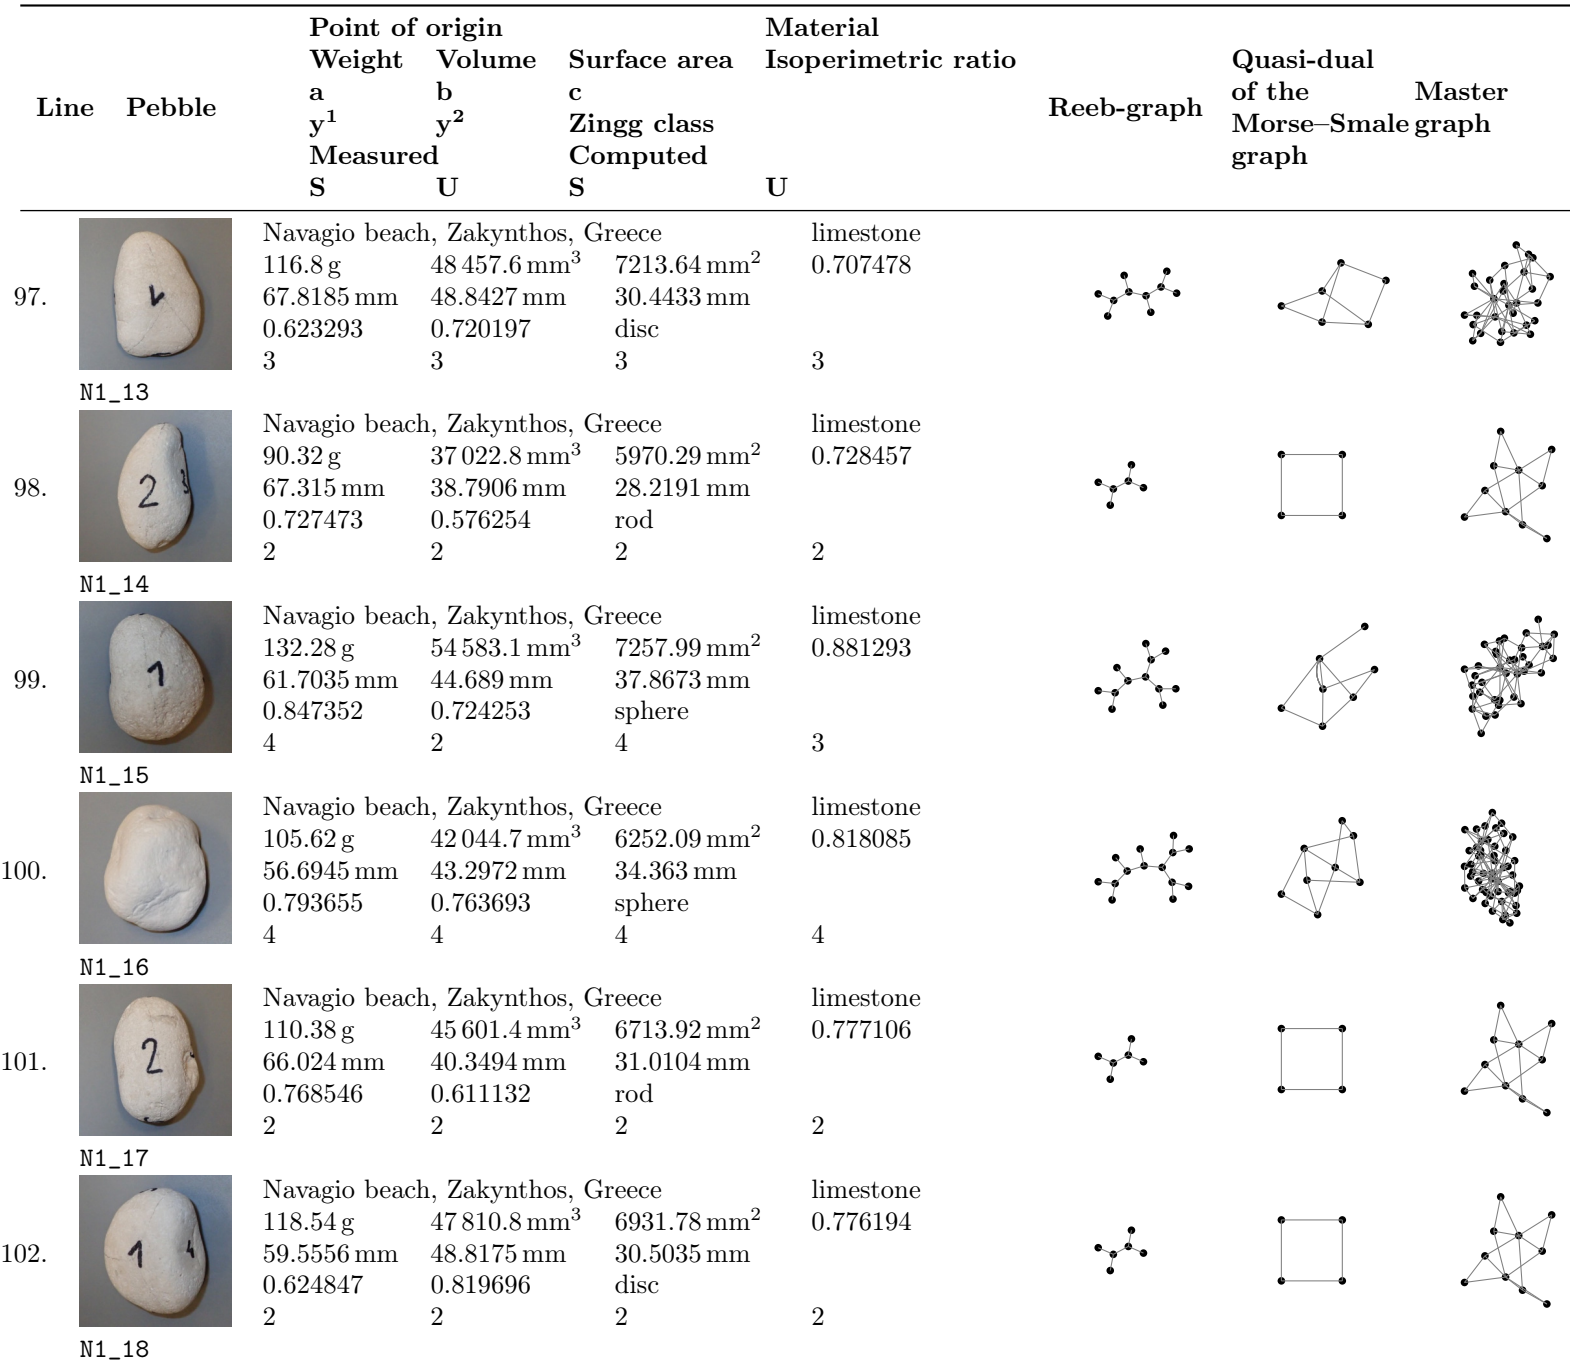   | 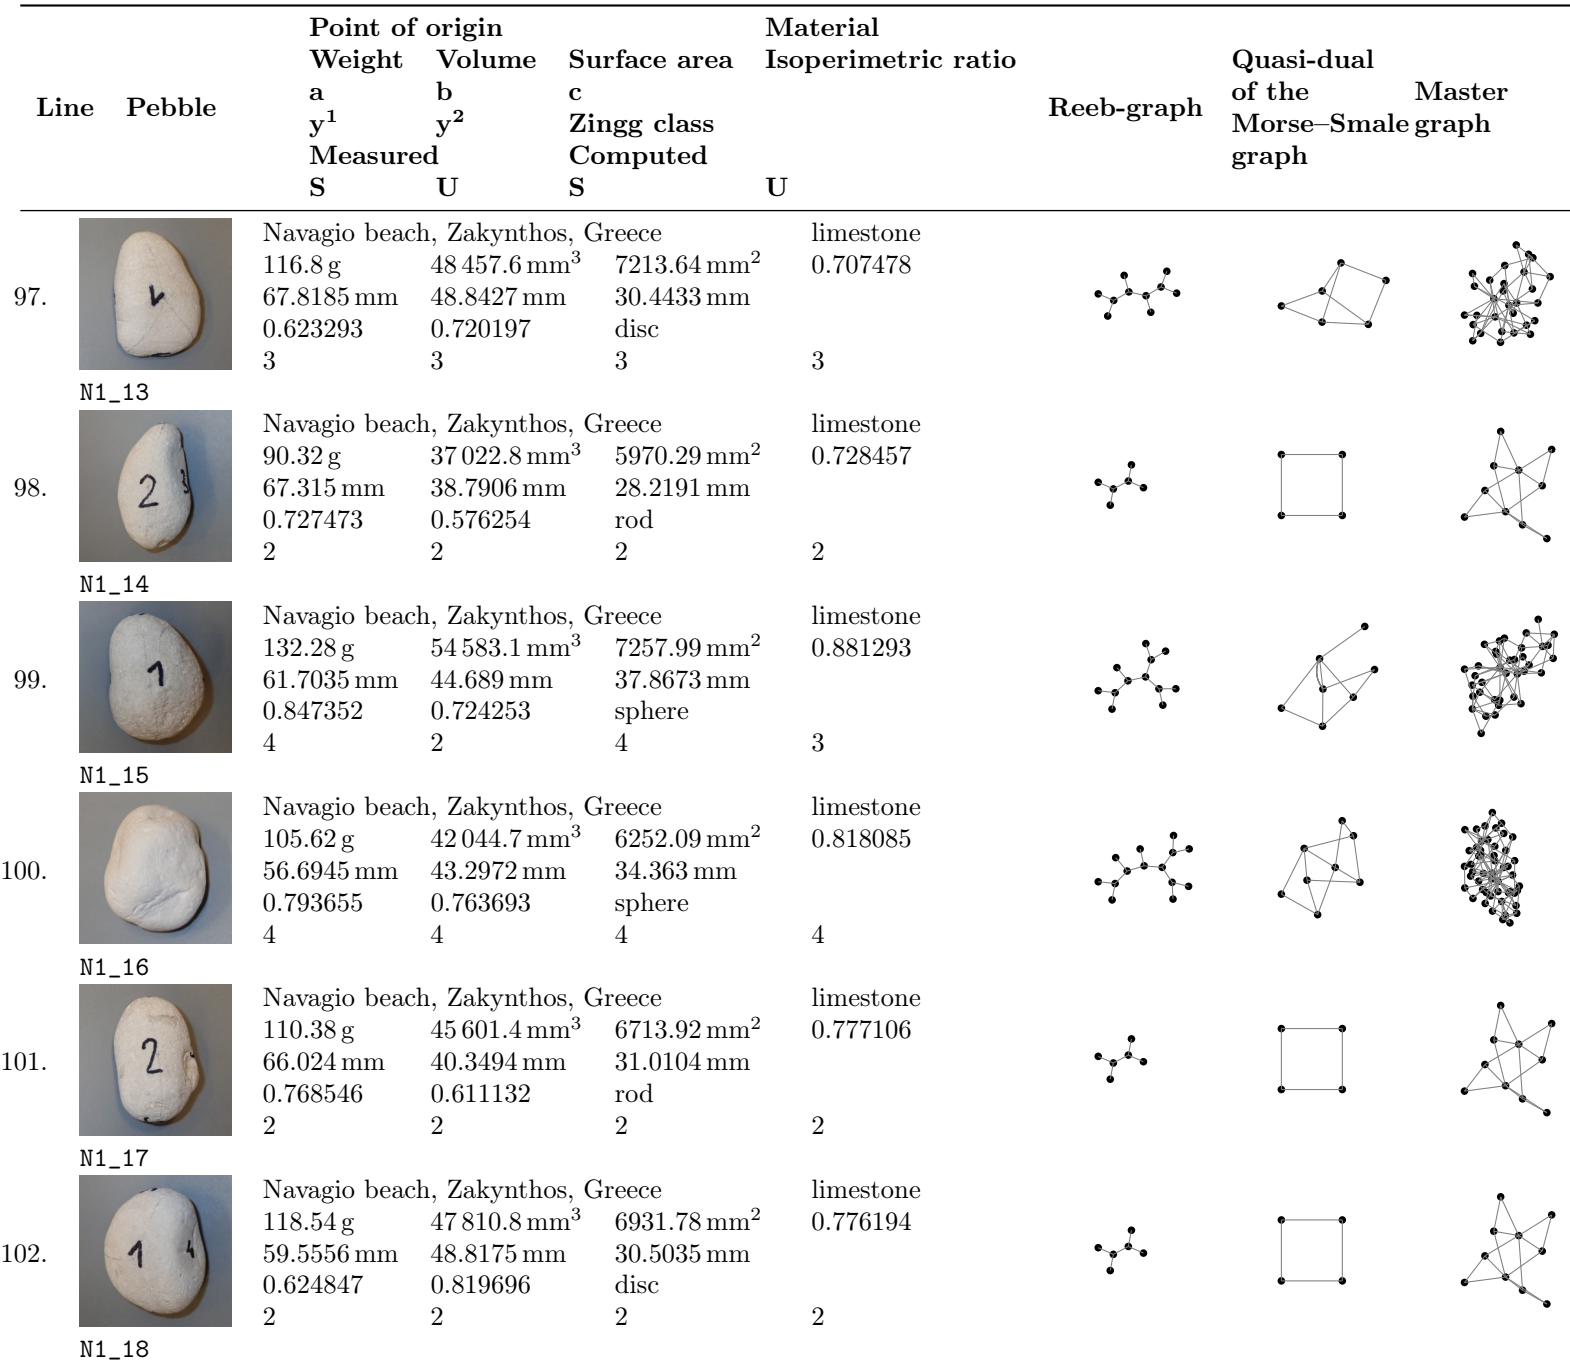   |
|      | N1_15                                                                               |                                                                             |                                                         |                                                      |                       |                                                                                       |                                                                                       |                                                                                       |
| 100. | 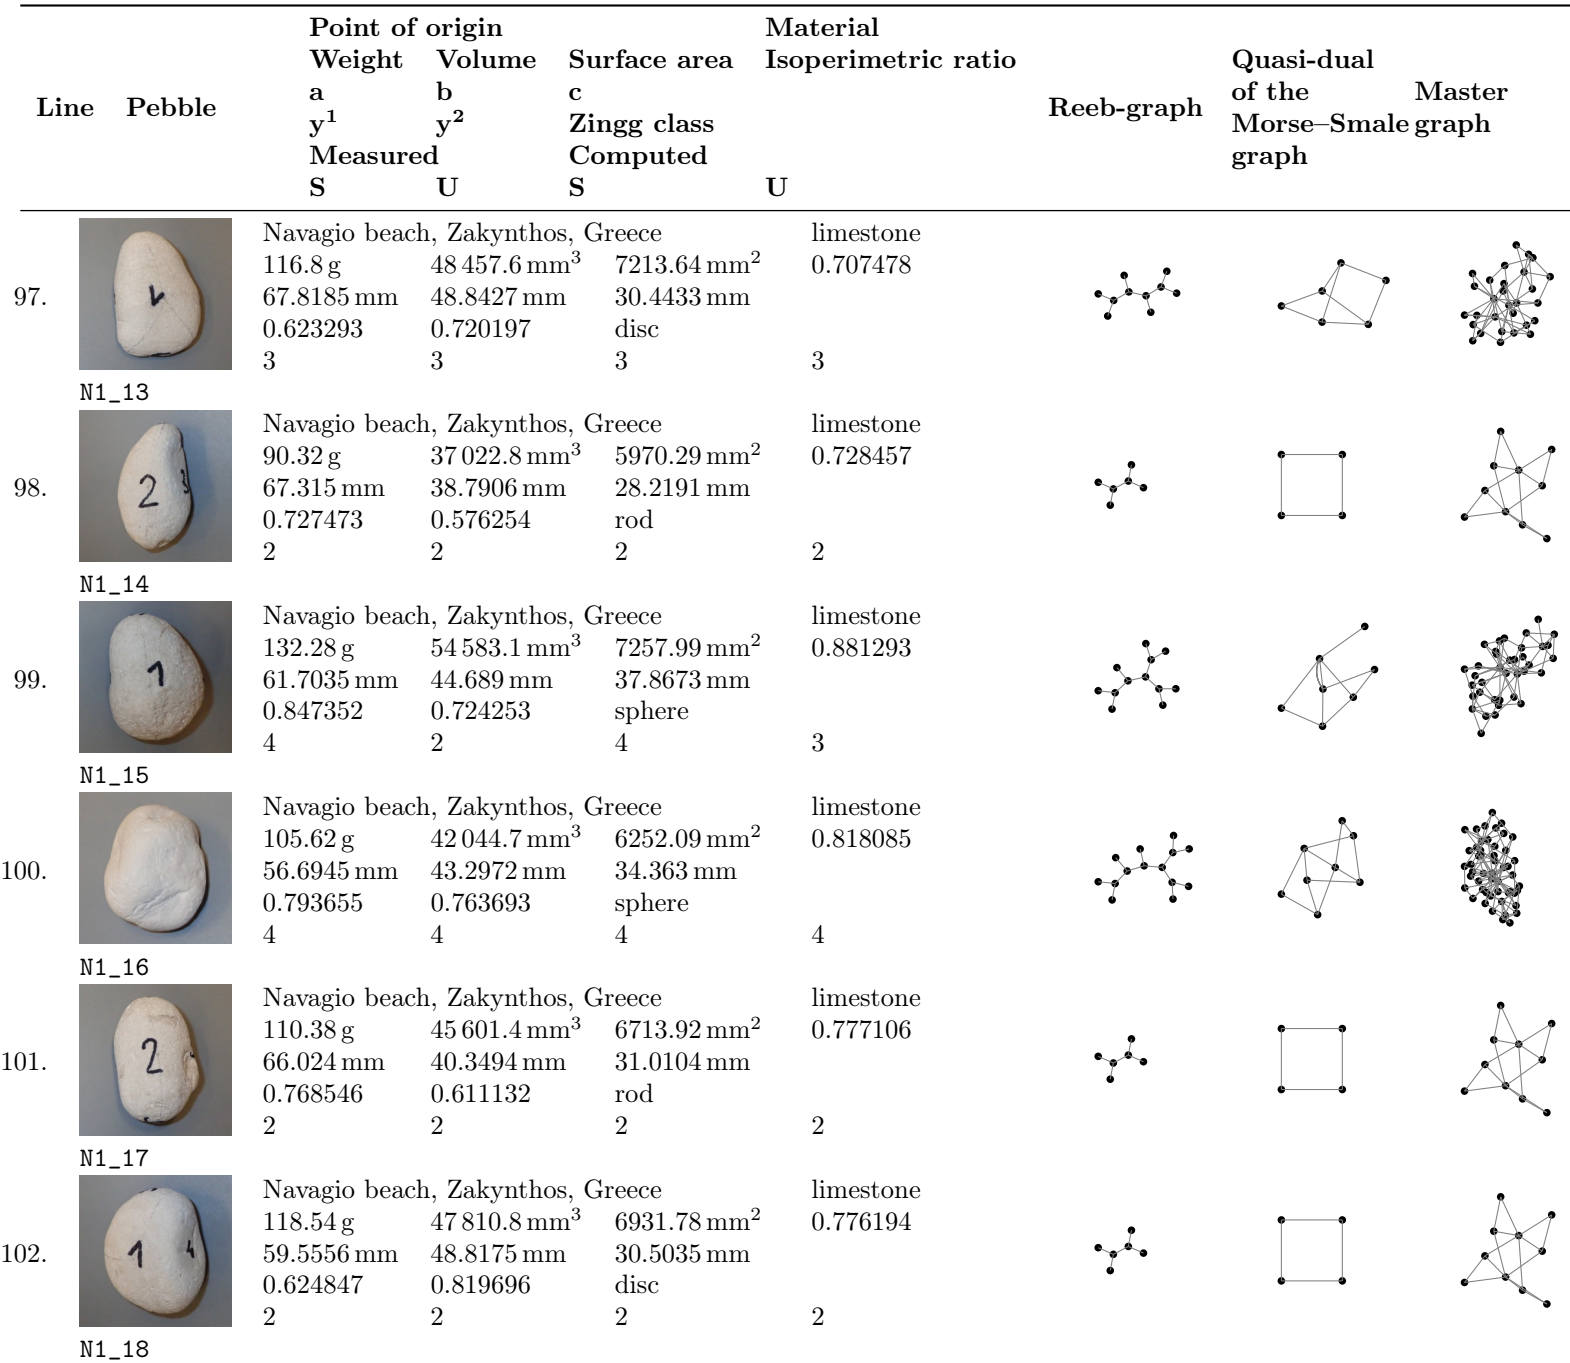  | Navagio beach, Zakynthos, Greece<br>105.62 g<br>56.6945 mm<br>0.793655<br>4 | 42 044.7 mm <sup>3</sup><br>43.2972 mm<br>0.763693<br>4 | 6252.09 mm <sup>2</sup><br>34.363 mm<br>sphere<br>4  | limestone<br>0.818085 | 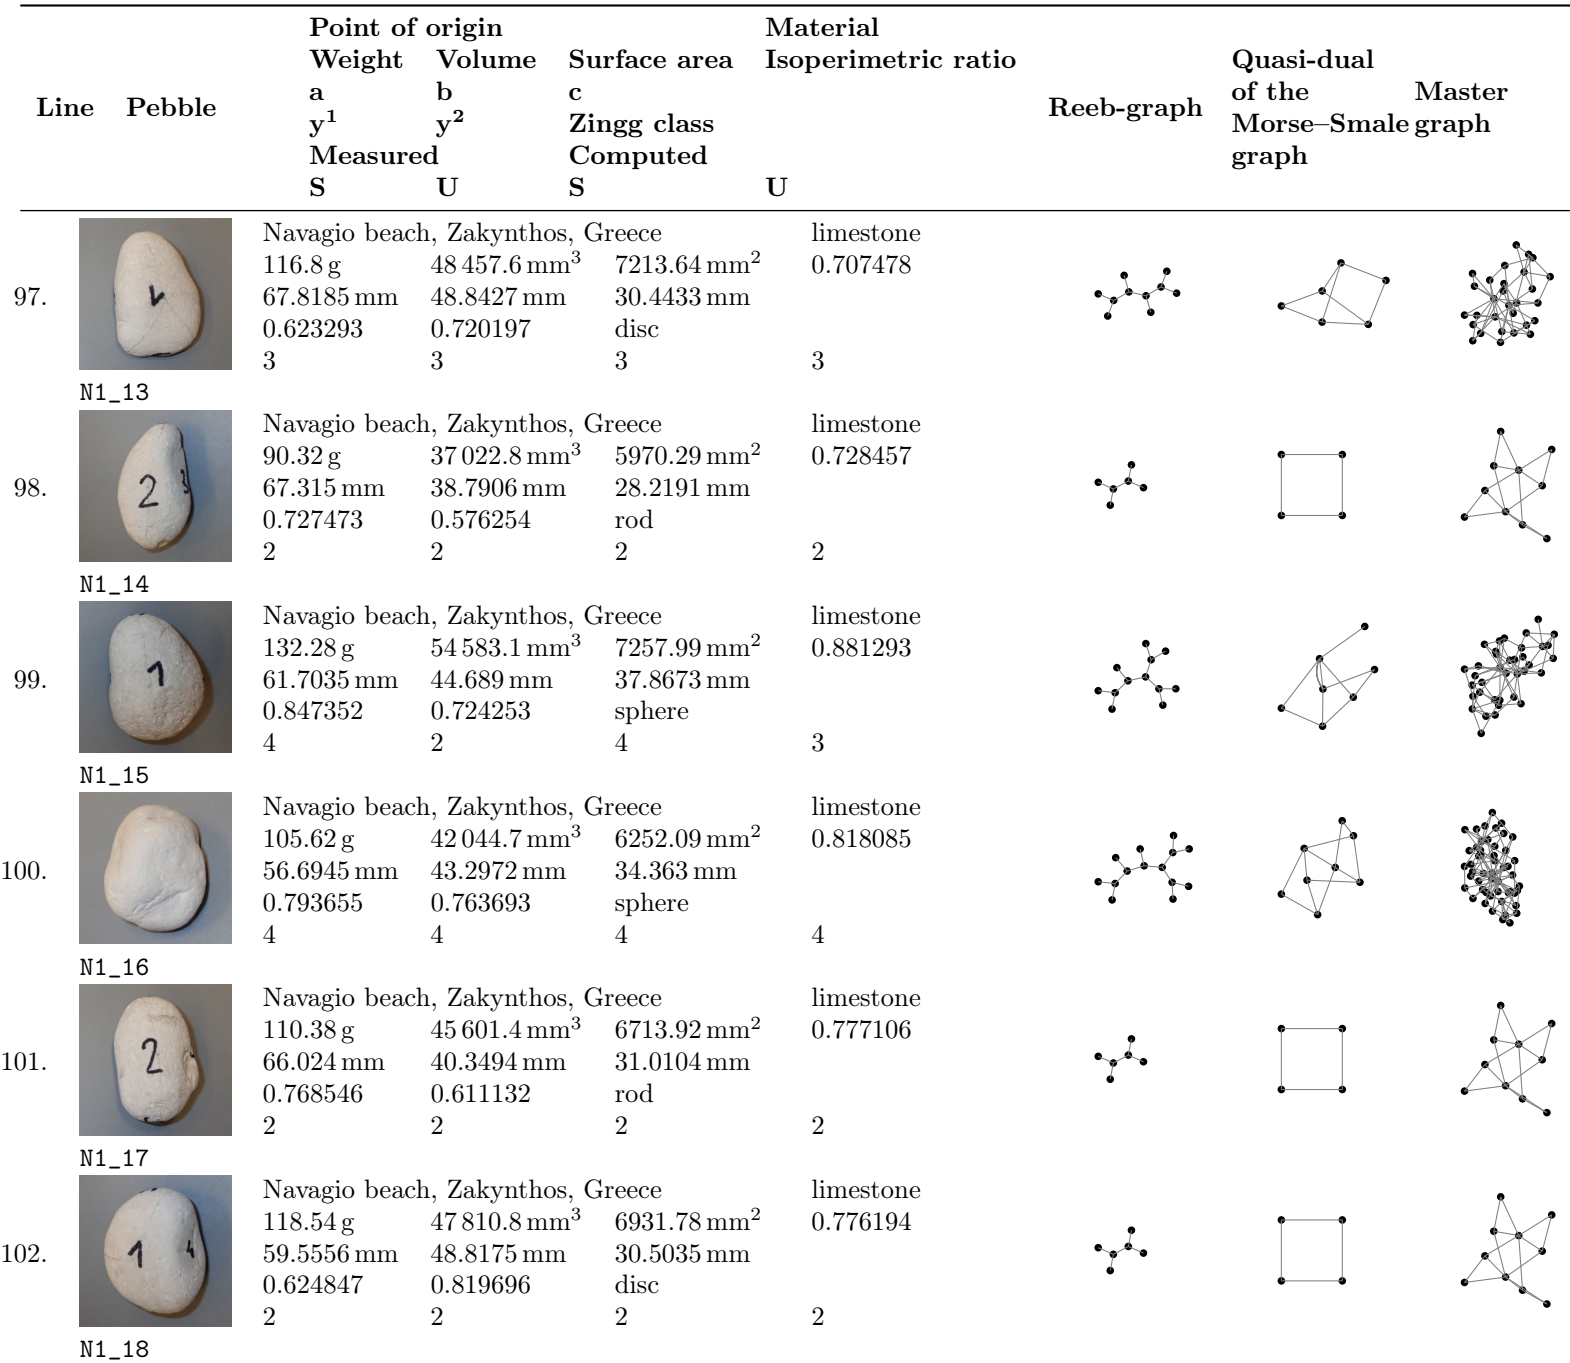  | 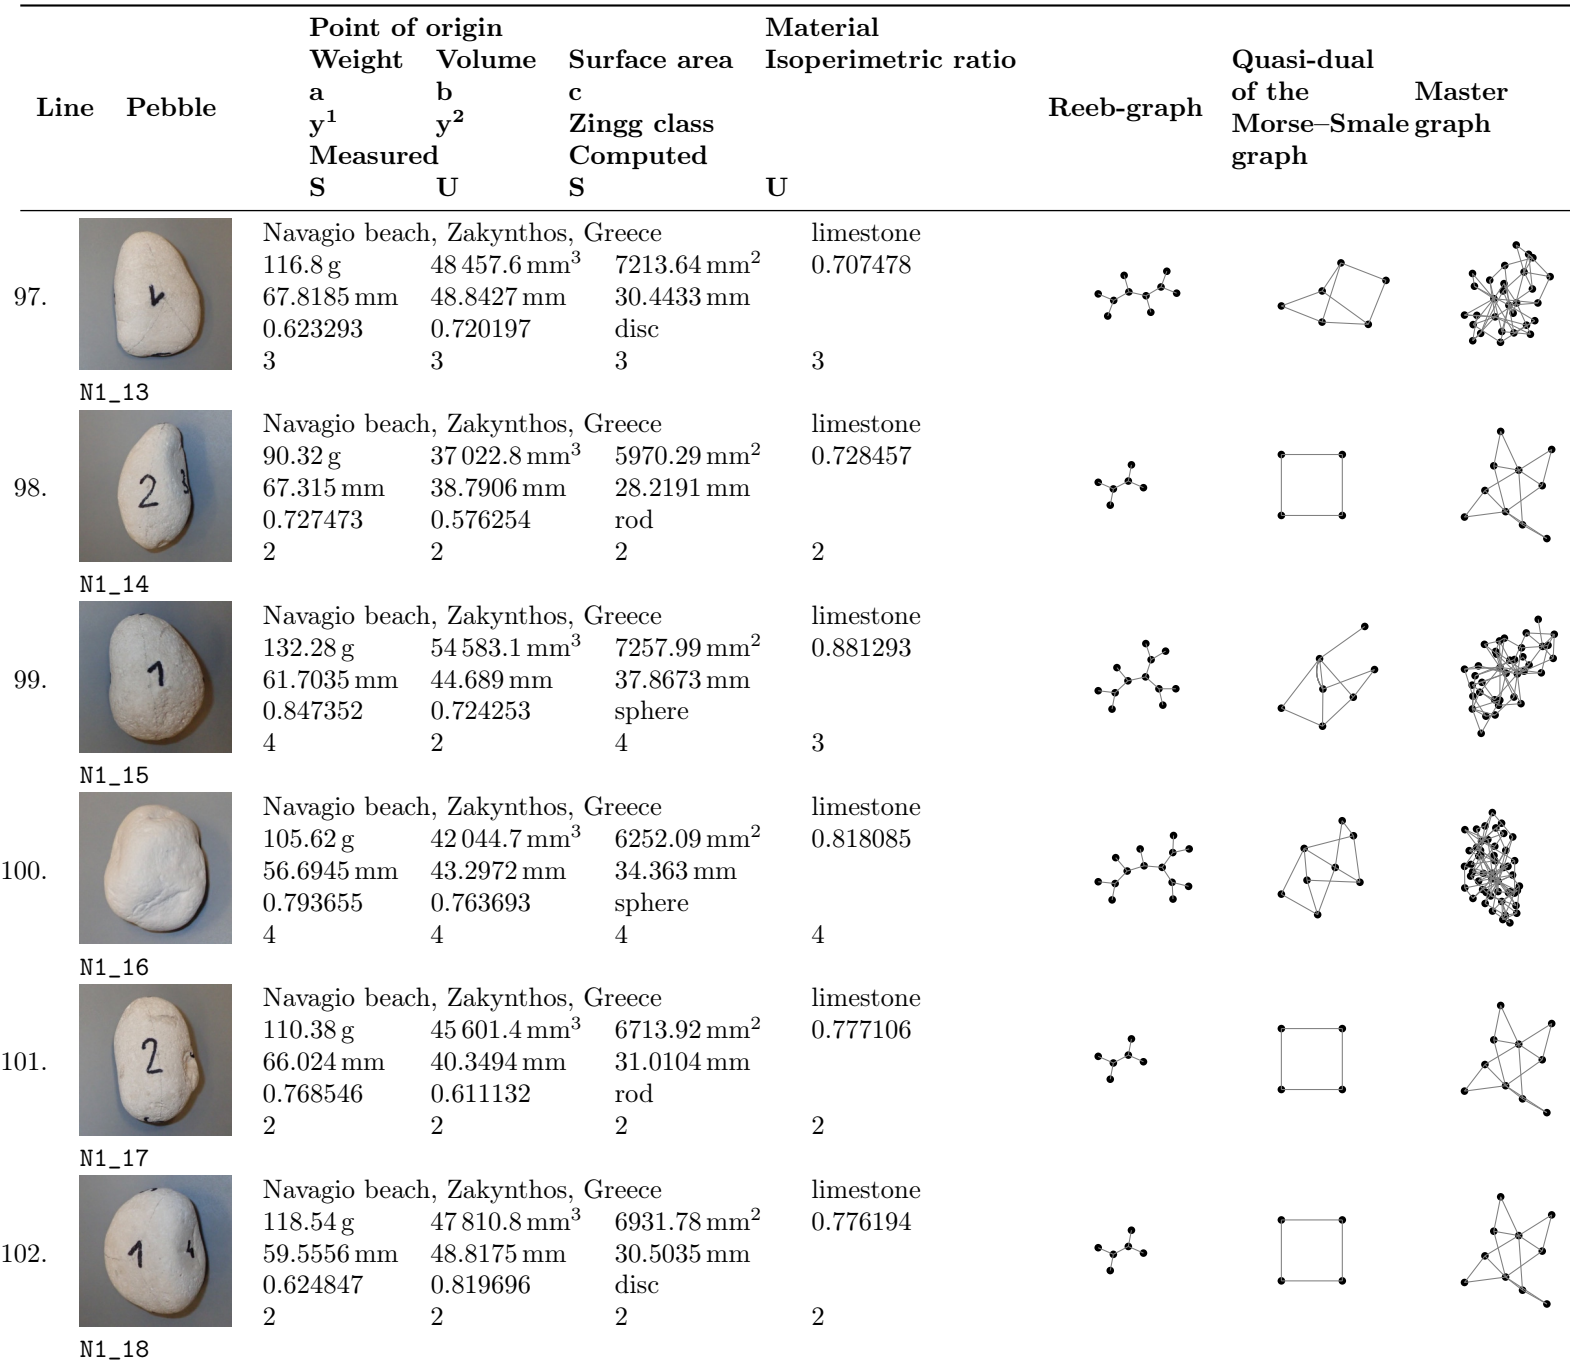  | 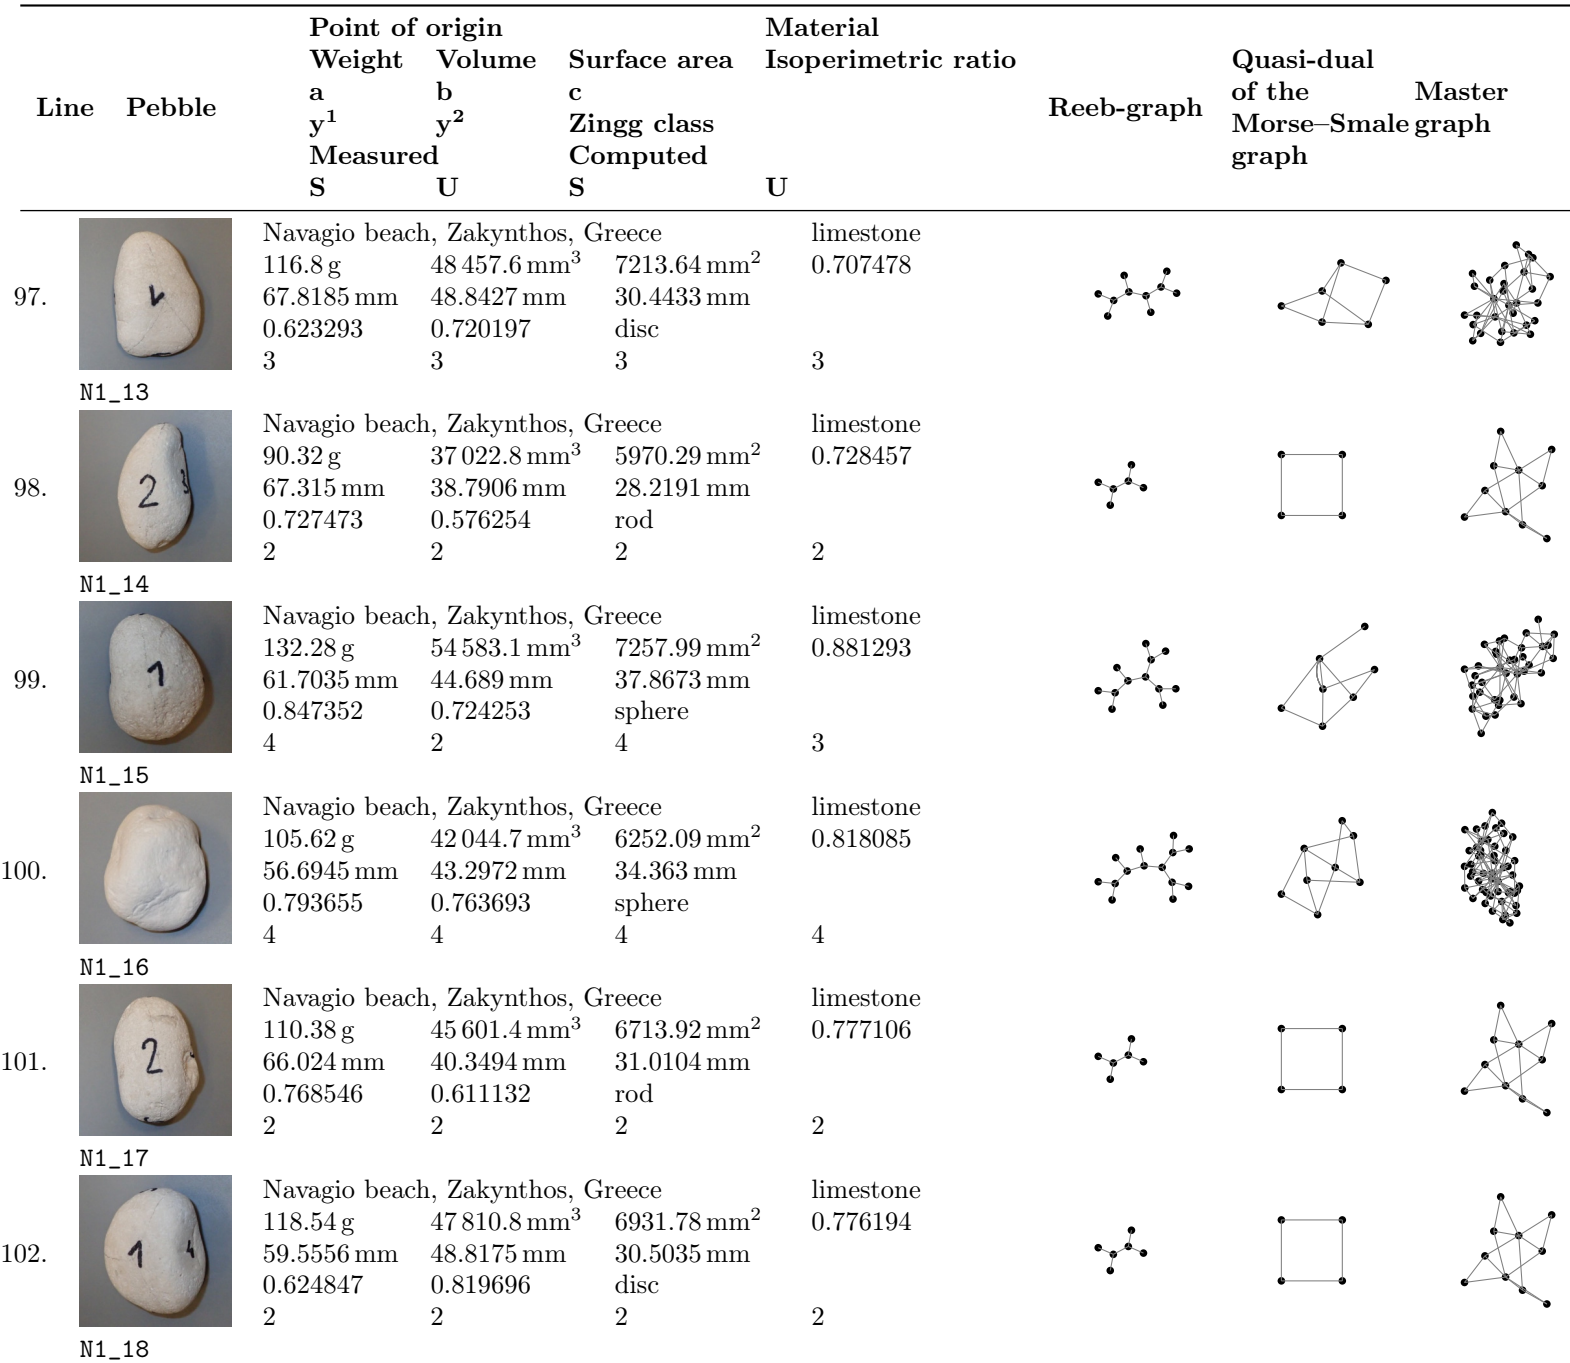  |
|      | N1_16                                                                               |                                                                             |                                                         |                                                      |                       |                                                                                       |                                                                                       |                                                                                       |
| 101. | 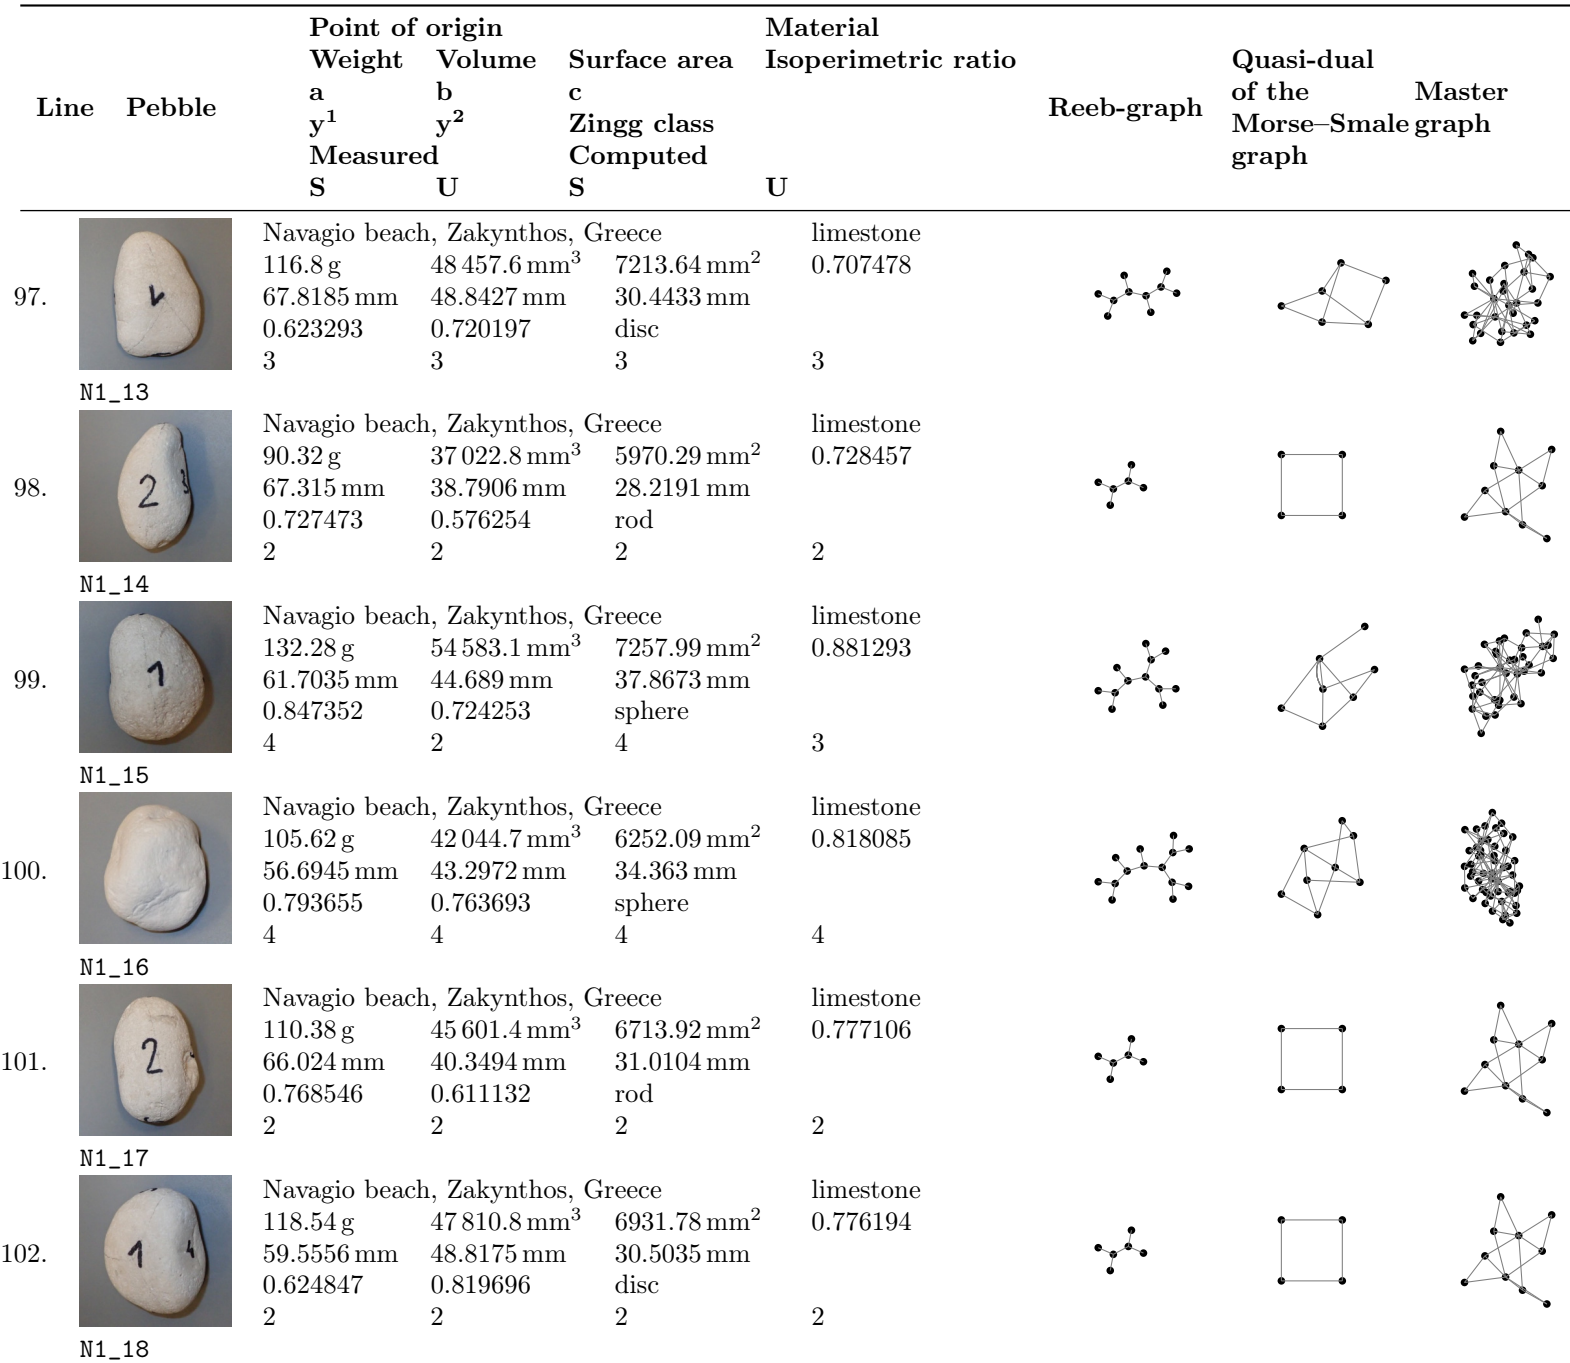 | Navagio beach, Zakynthos, Greece<br>110.38 g<br>66.024 mm<br>0.768546<br>2  | 45 601.4 mm <sup>3</sup><br>40.3494 mm<br>0.611132<br>2 | 6713.92 mm <sup>2</sup><br>31.0104 mm<br>rod<br>2    | limestone<br>0.777106 | 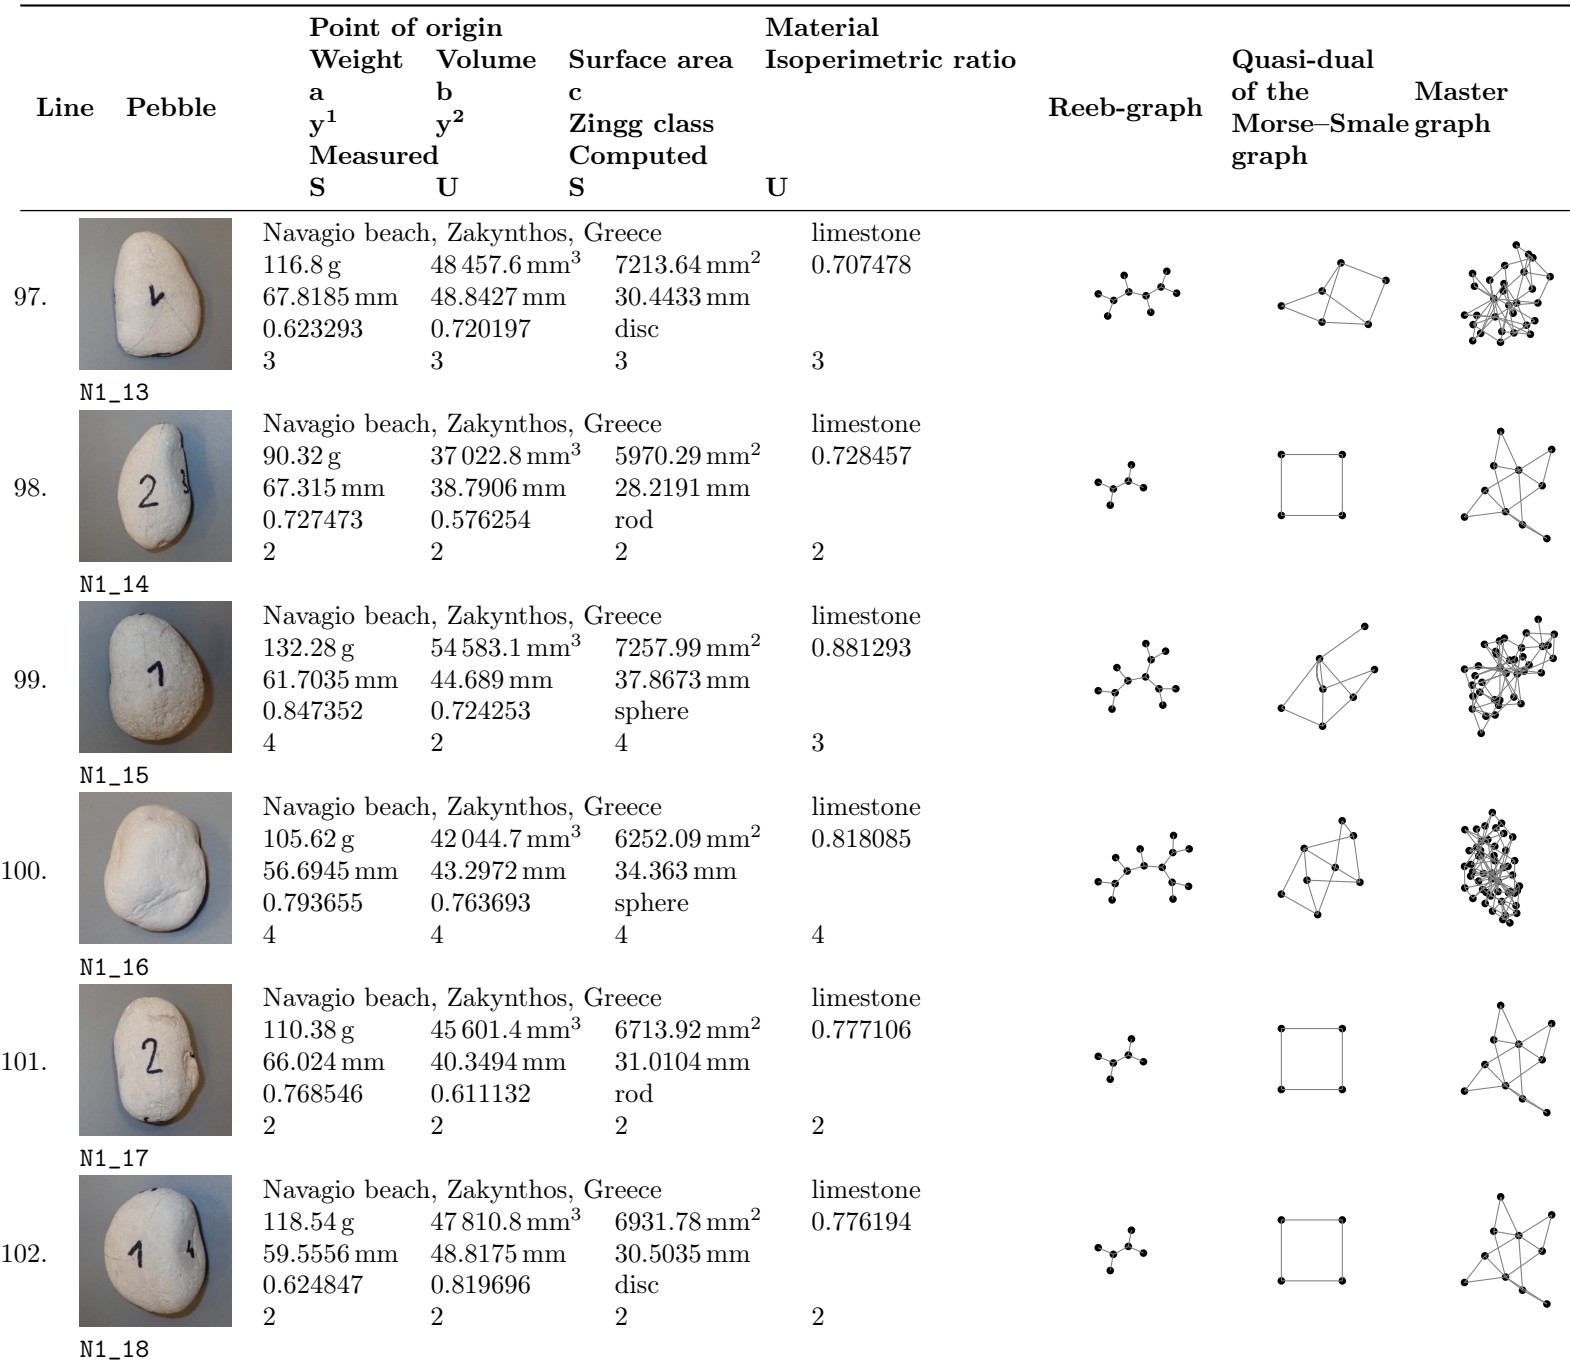 | 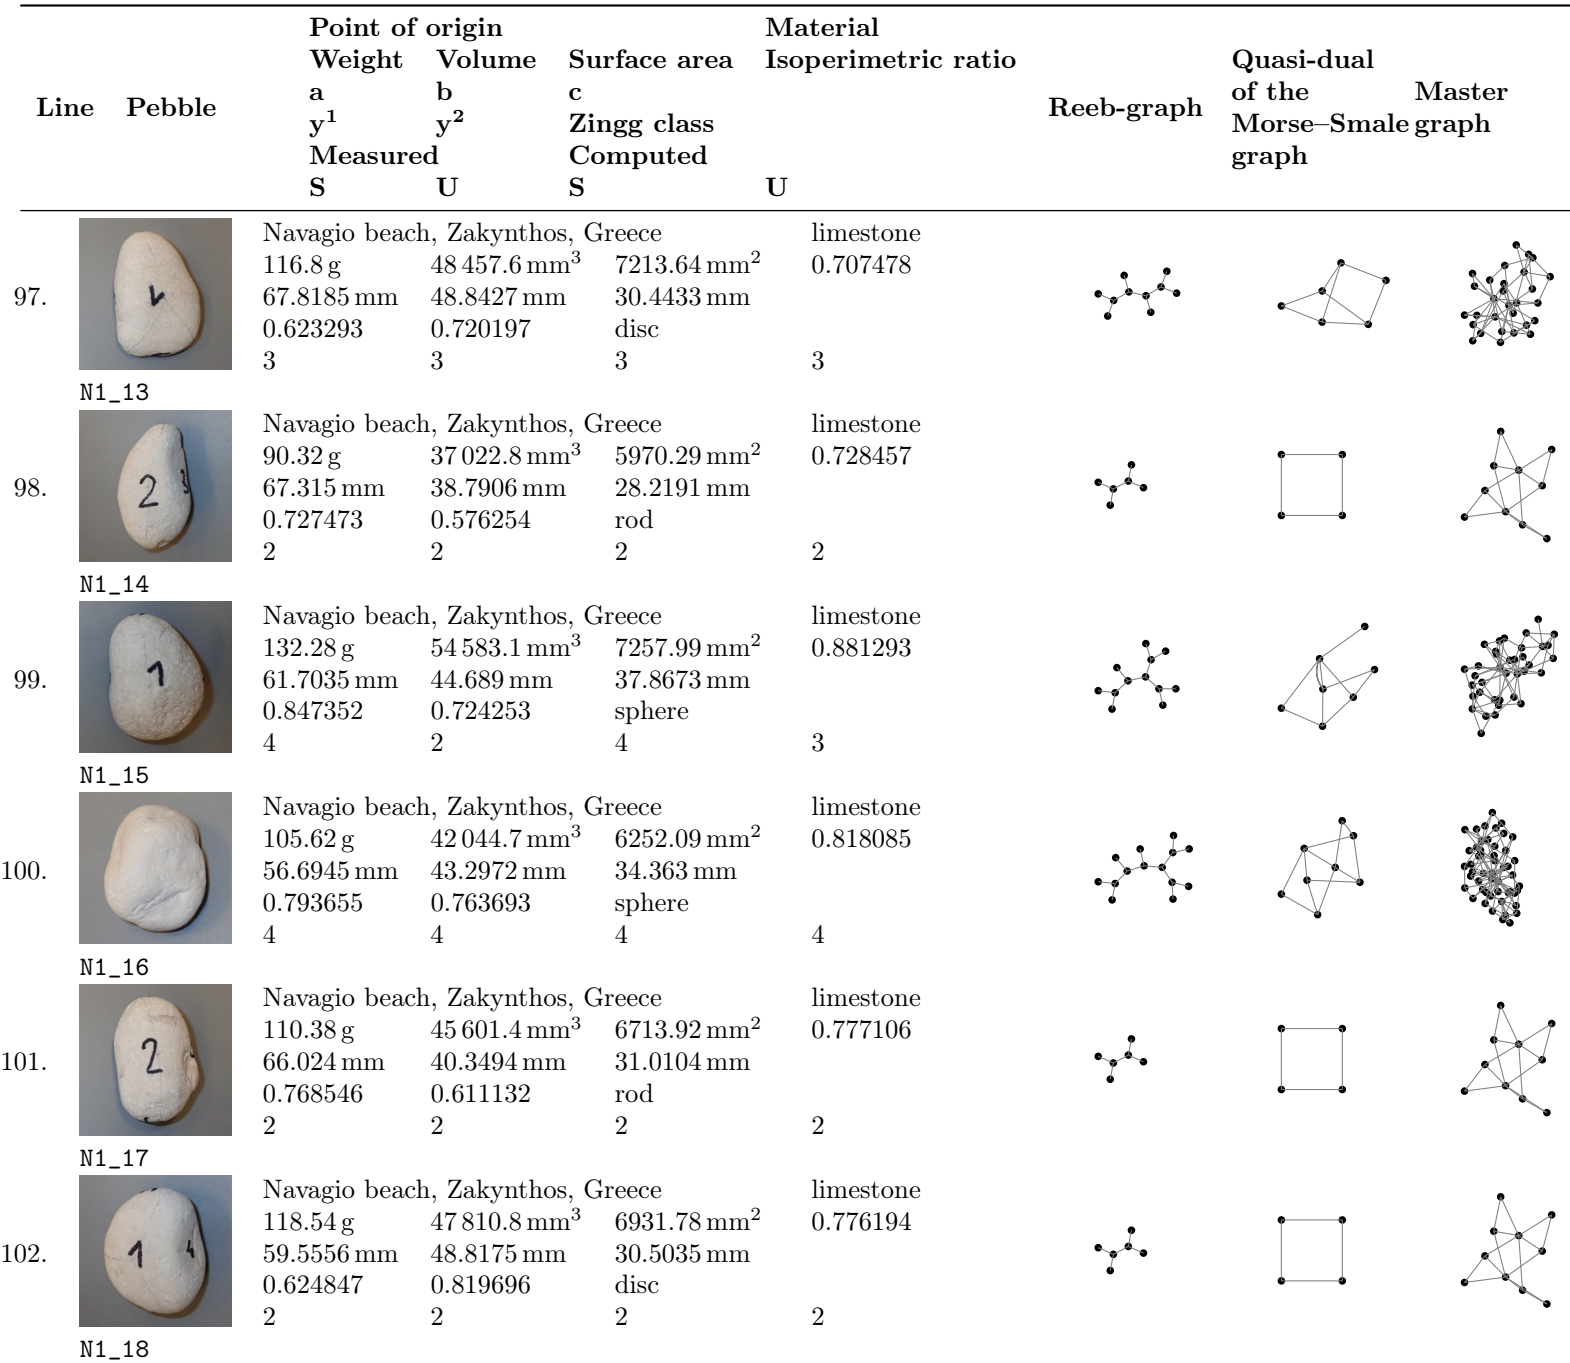 | 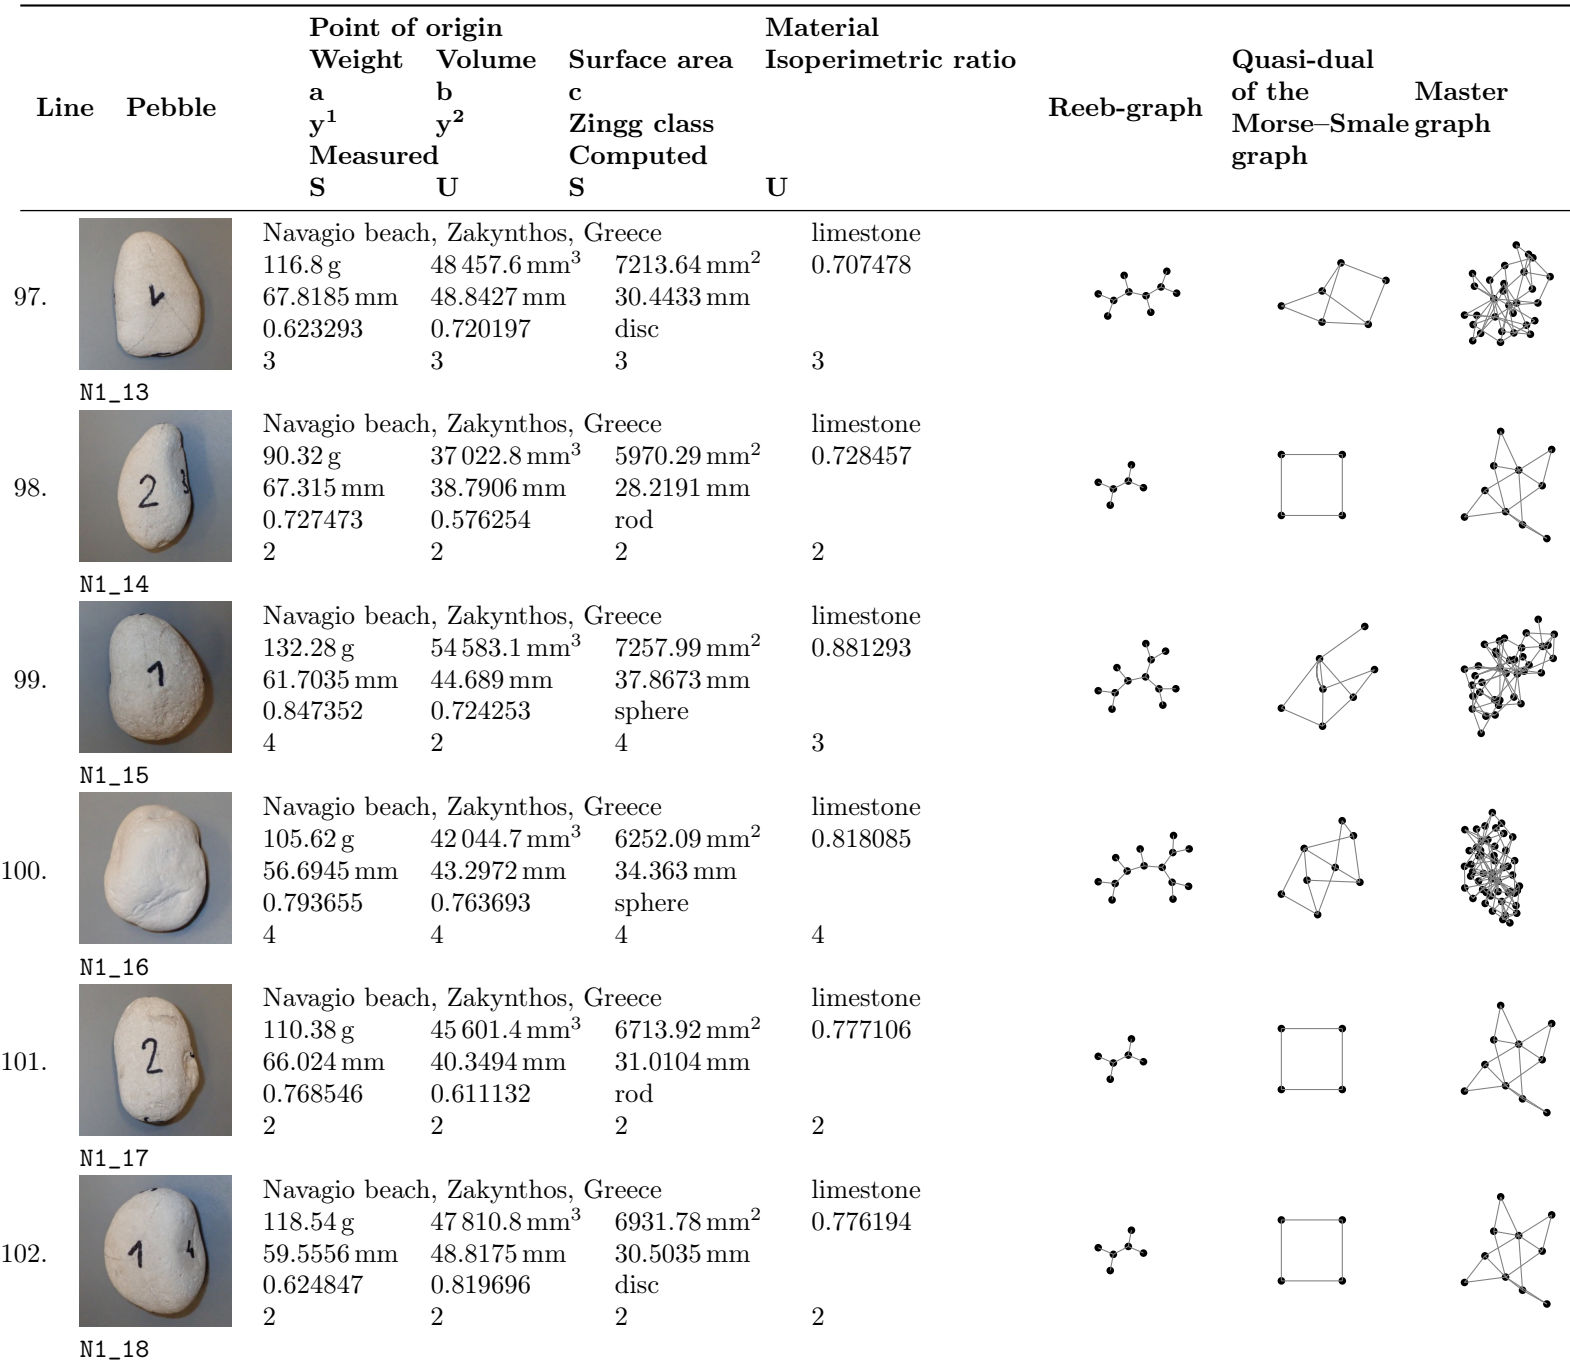 |
|      | N1_17                                                                               |                                                                             |                                                         |                                                      |                       |                                                                                       |                                                                                       |                                                                                       |
| 102. | 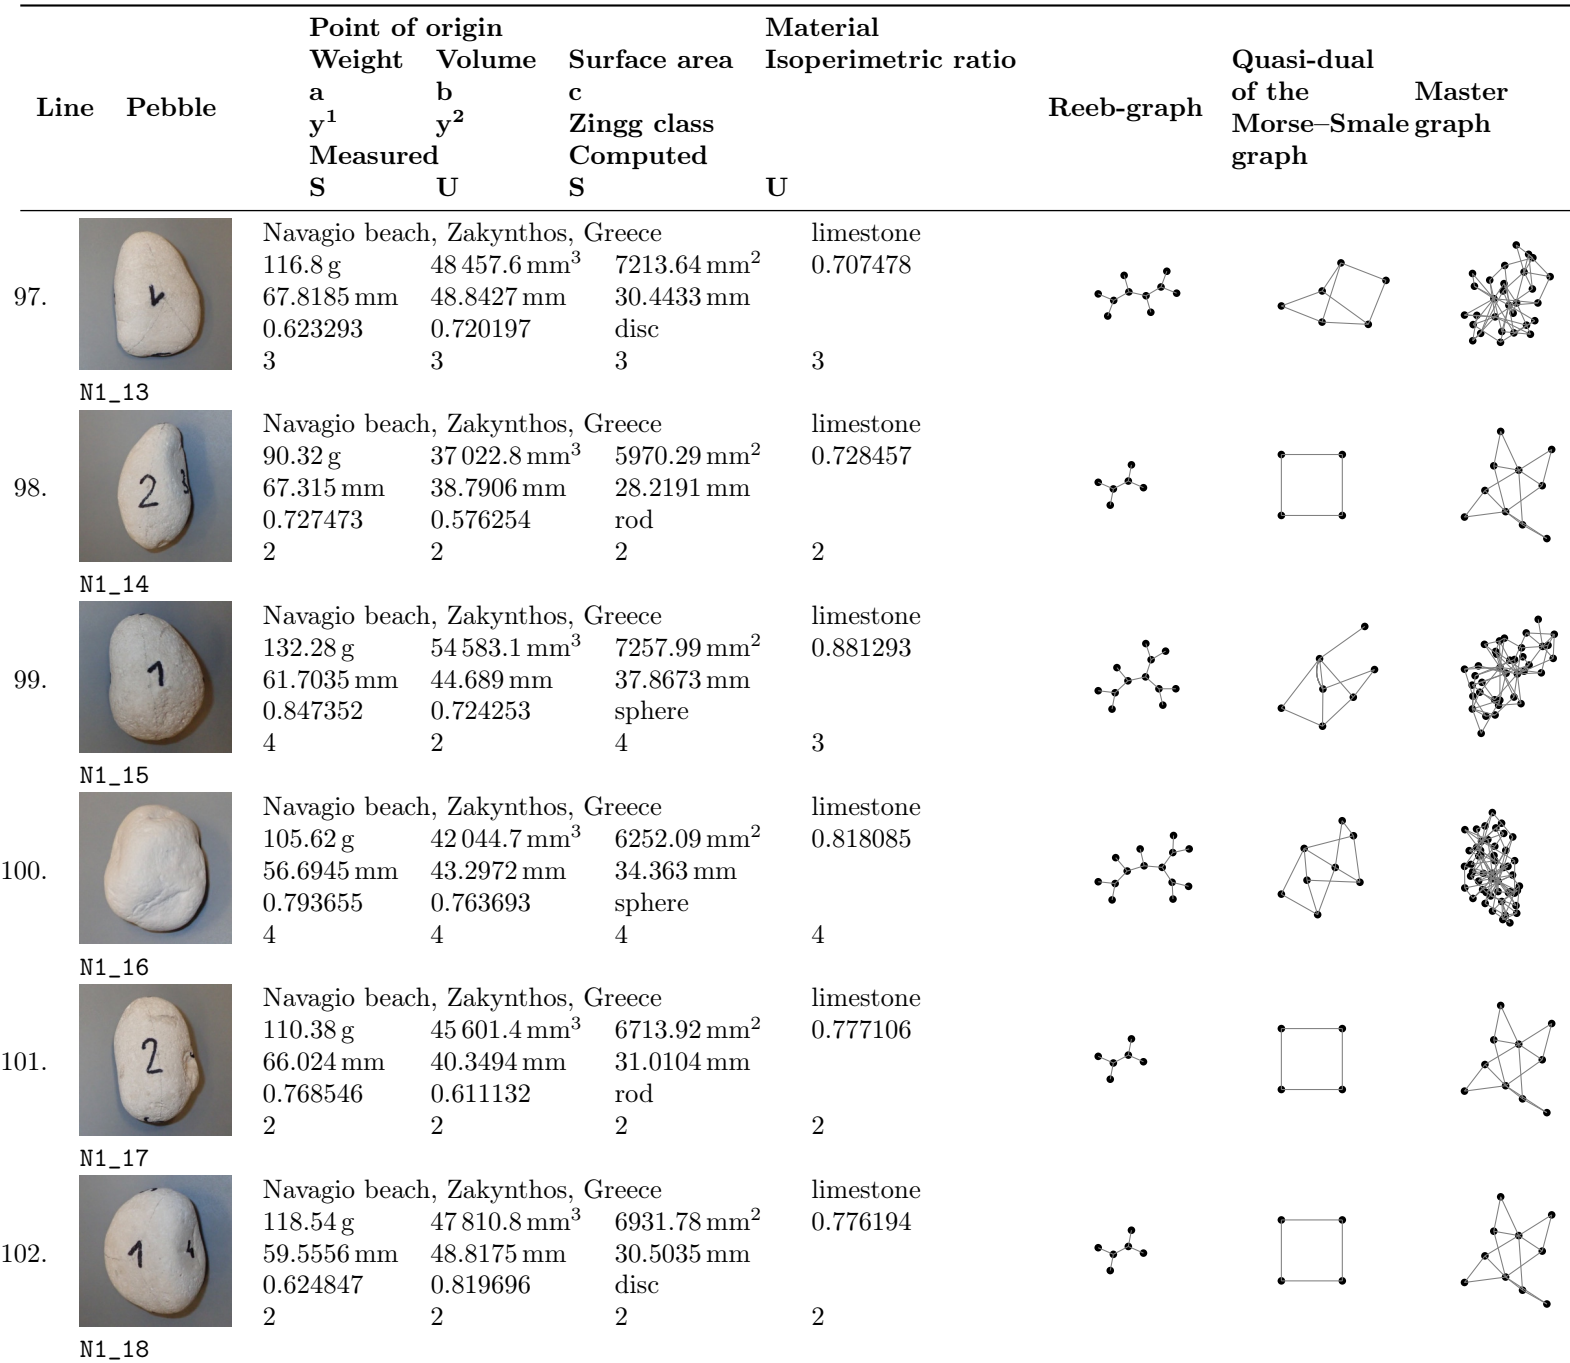 | Navagio beach, Zakynthos, Greece<br>118.54 g<br>59.5556 mm<br>0.624847<br>2 | 47 810.8 mm <sup>3</sup><br>48.8175 mm<br>0.819696<br>2 | 6931.78 mm <sup>2</sup><br>30.5035 mm<br>disc<br>2   | limestone<br>0.776194 | 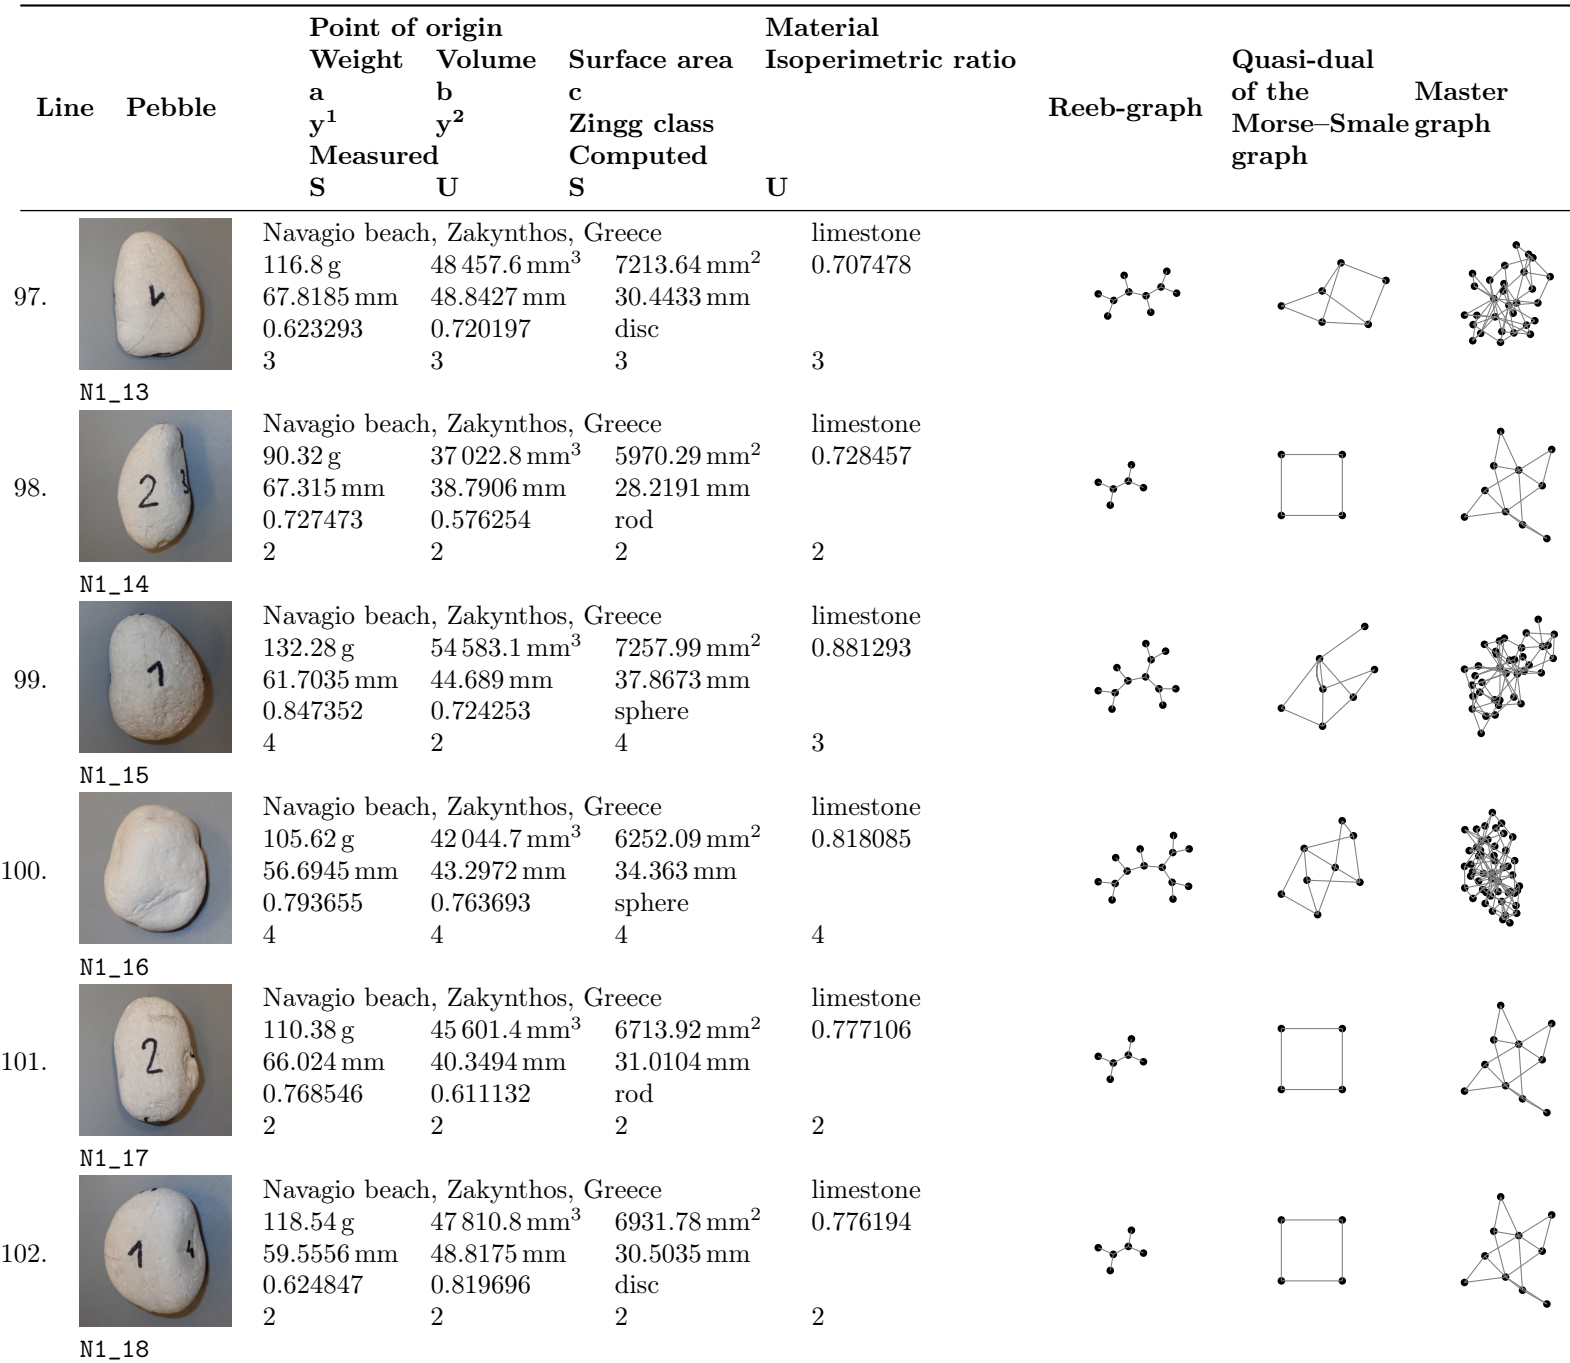 | 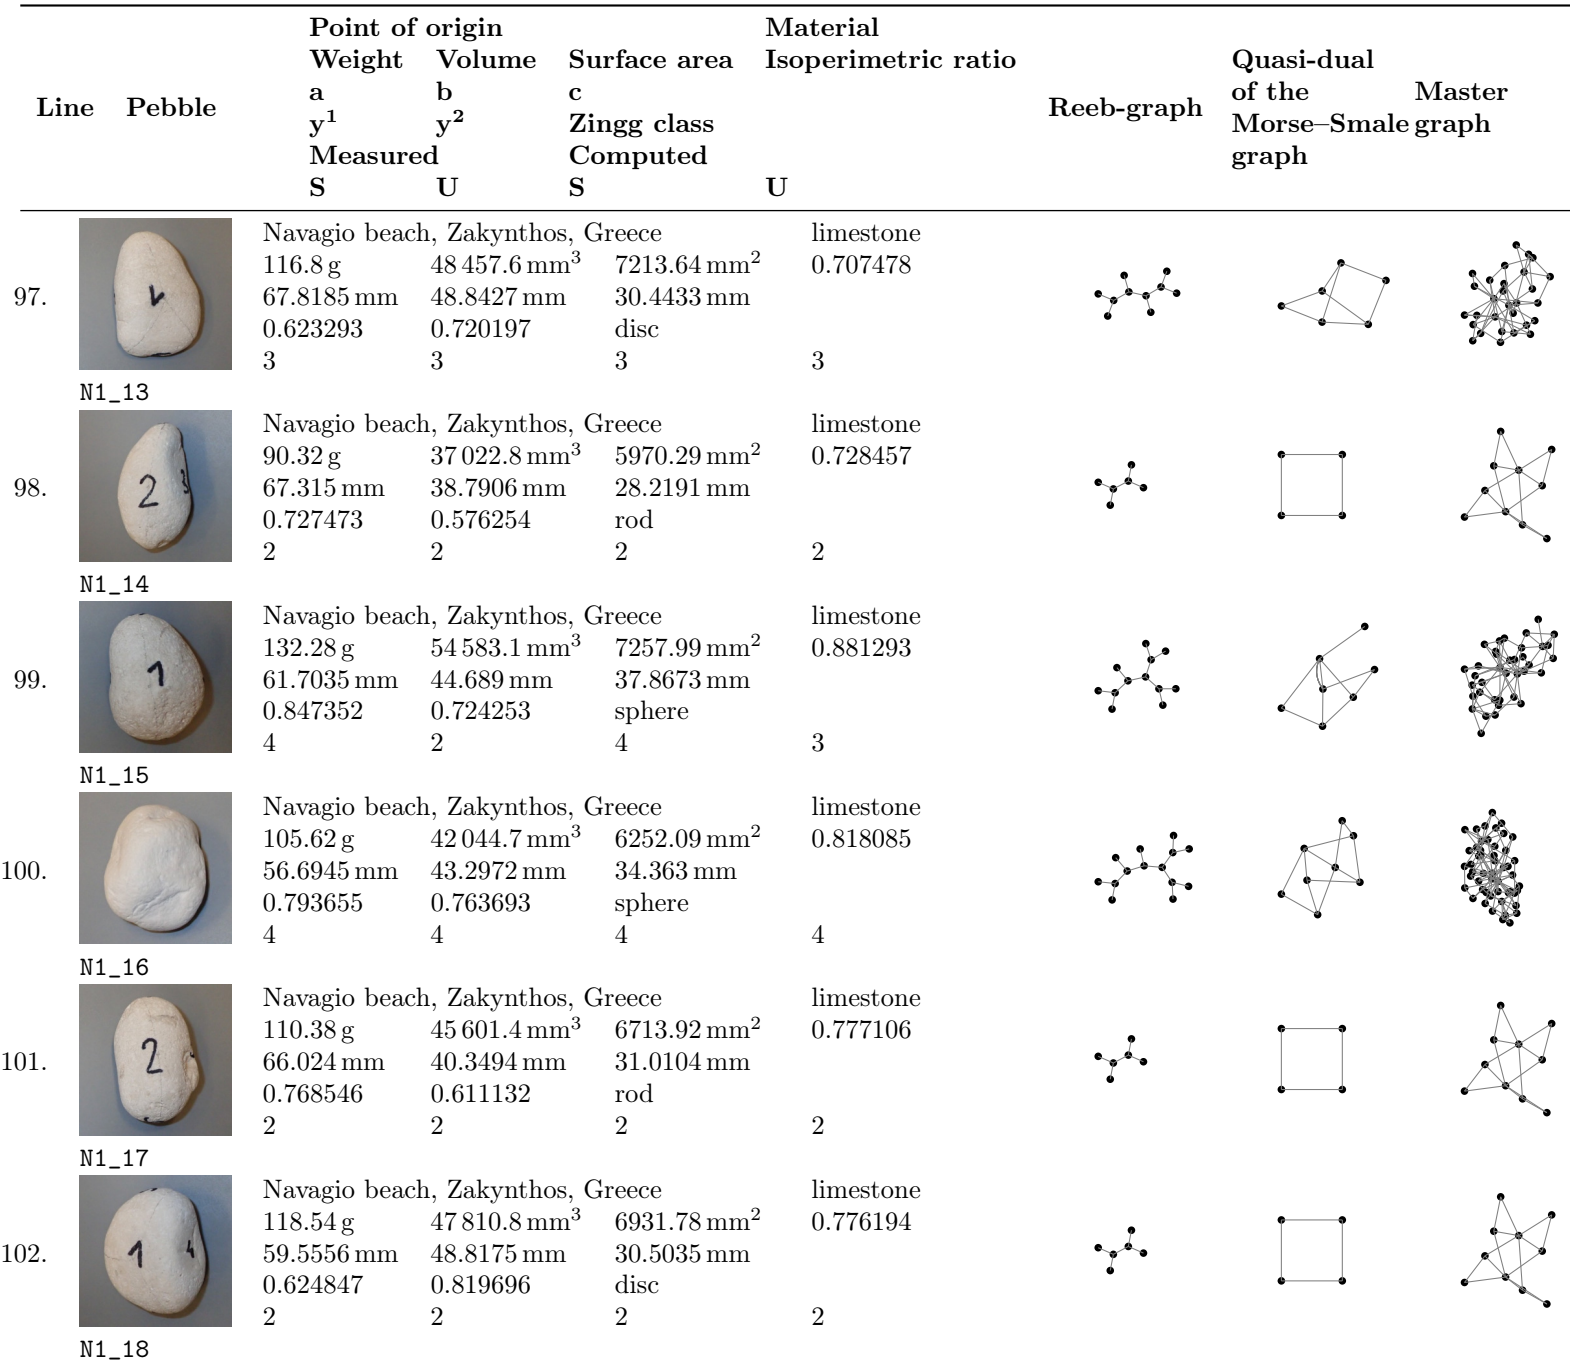 | 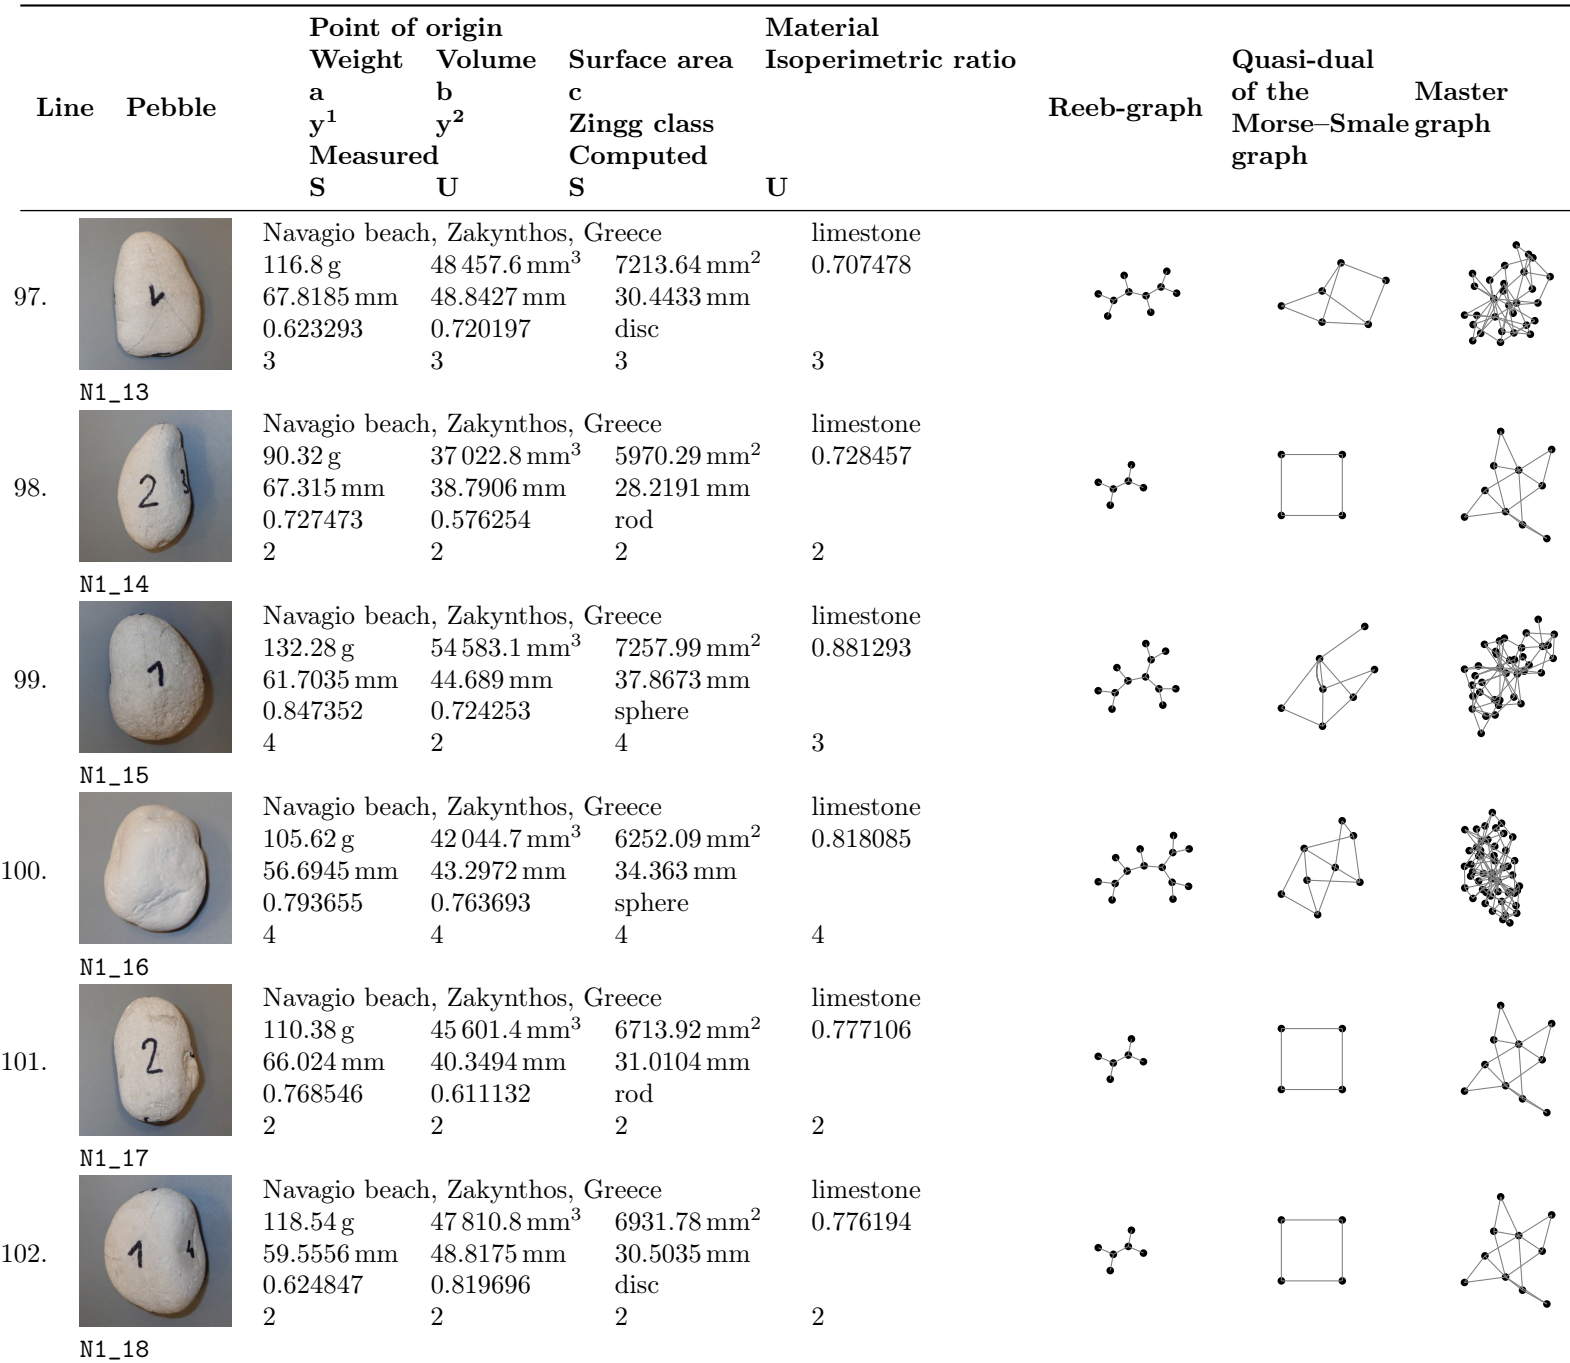 |
|      | N1_18                                                                               |                                                                             |                                                         |                                                      |                       |                                                                                       |                                                                                       |                                                                                       |

| Line | Pebble                                                                              | Point of origin                  |                          |                              | Material  | Isoperimetric ratio | Reeb-graph                                                                            | Quasi-dual<br>of the<br>Morse–Smale<br>graph                                          | Master<br>graph                                                                       |
|------|-------------------------------------------------------------------------------------|----------------------------------|--------------------------|------------------------------|-----------|---------------------|---------------------------------------------------------------------------------------|---------------------------------------------------------------------------------------|---------------------------------------------------------------------------------------|
|      |                                                                                     | Weight                           | Volume                   | Surface area                 |           |                     |                                                                                       |                                                                                       |                                                                                       |
|      |                                                                                     | a                                | b                        | c                            |           |                     |                                                                                       |                                                                                       |                                                                                       |
|      |                                                                                     | y <sup>1</sup><br>Measured<br>S  | y <sup>2</sup><br>U      | Zingg class<br>Computed<br>S |           |                     |                                                                                       |                                                                                       |                                                                                       |
| 103. | 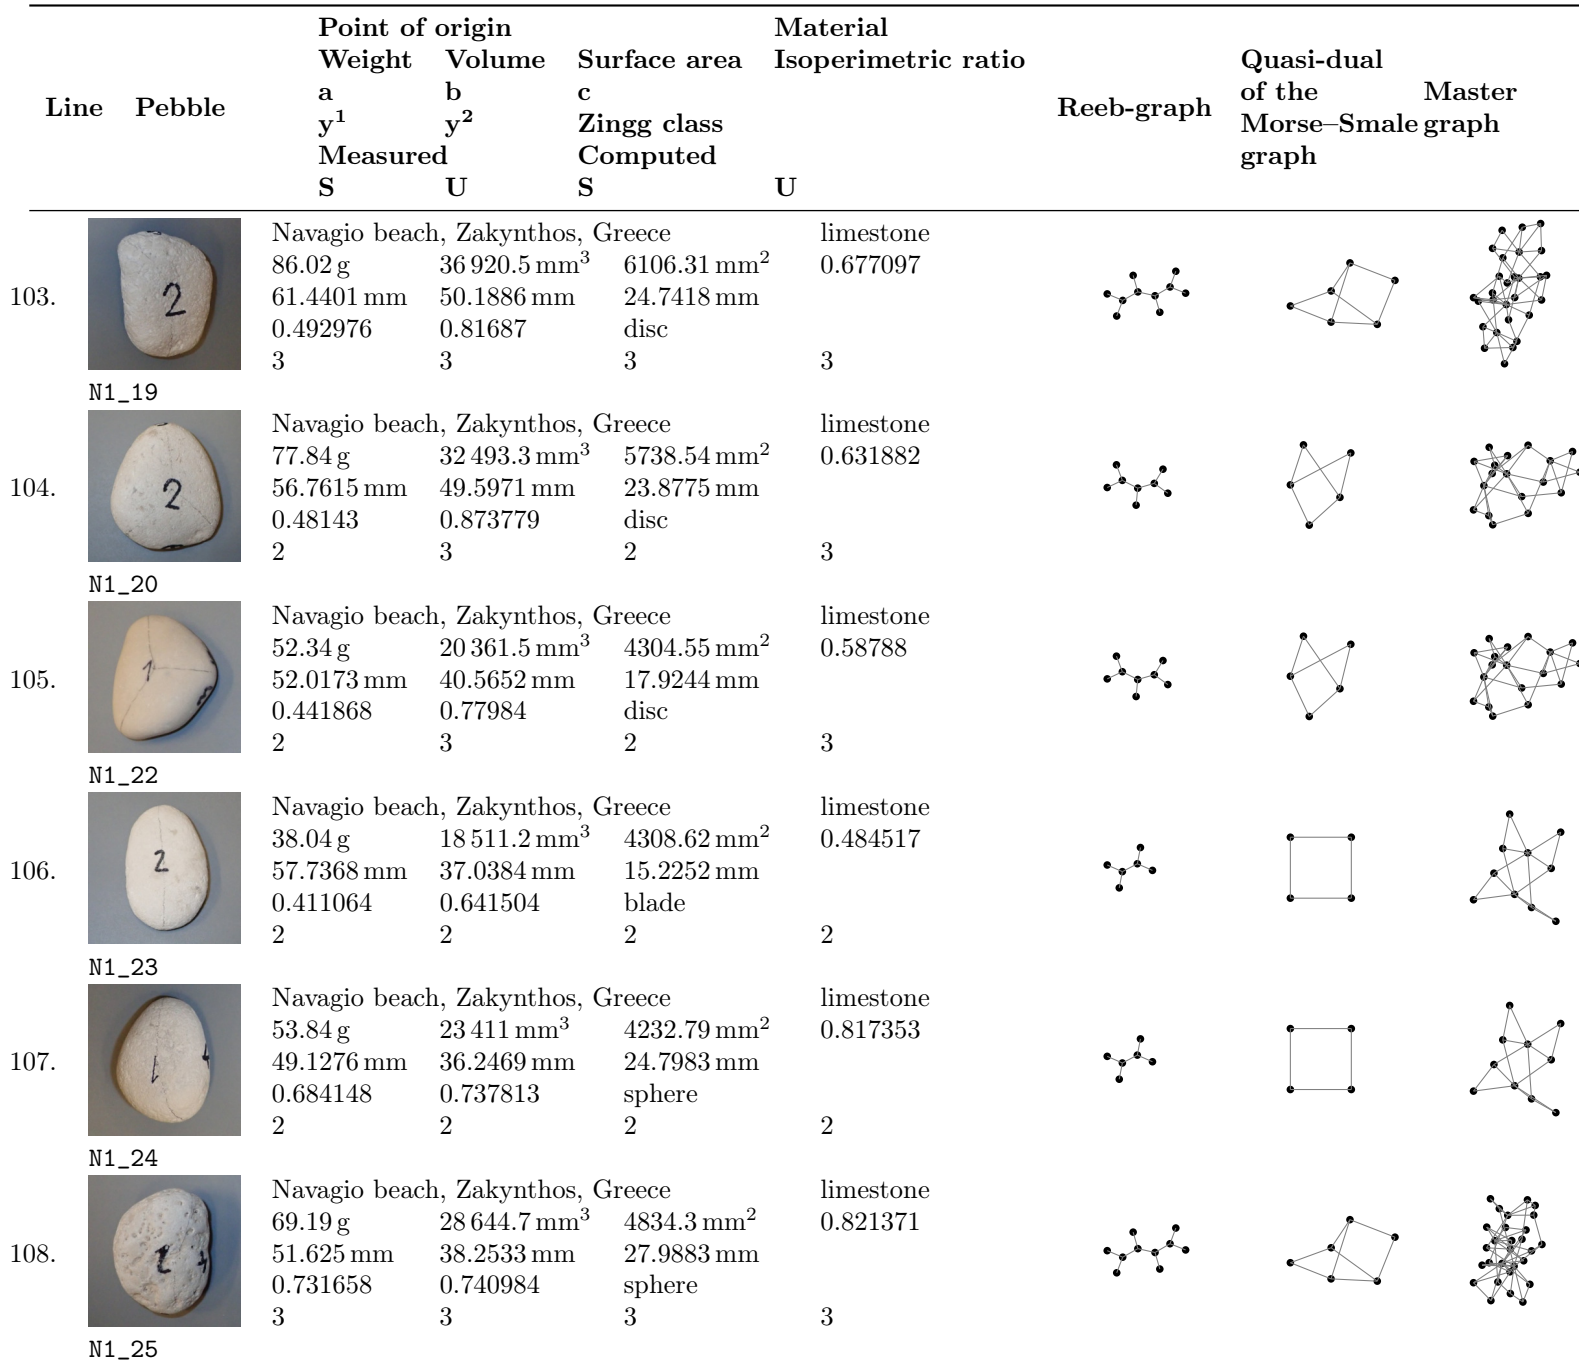   | Navagio beach, Zakynthos, Greece |                          |                              | limestone | 0.677097            | 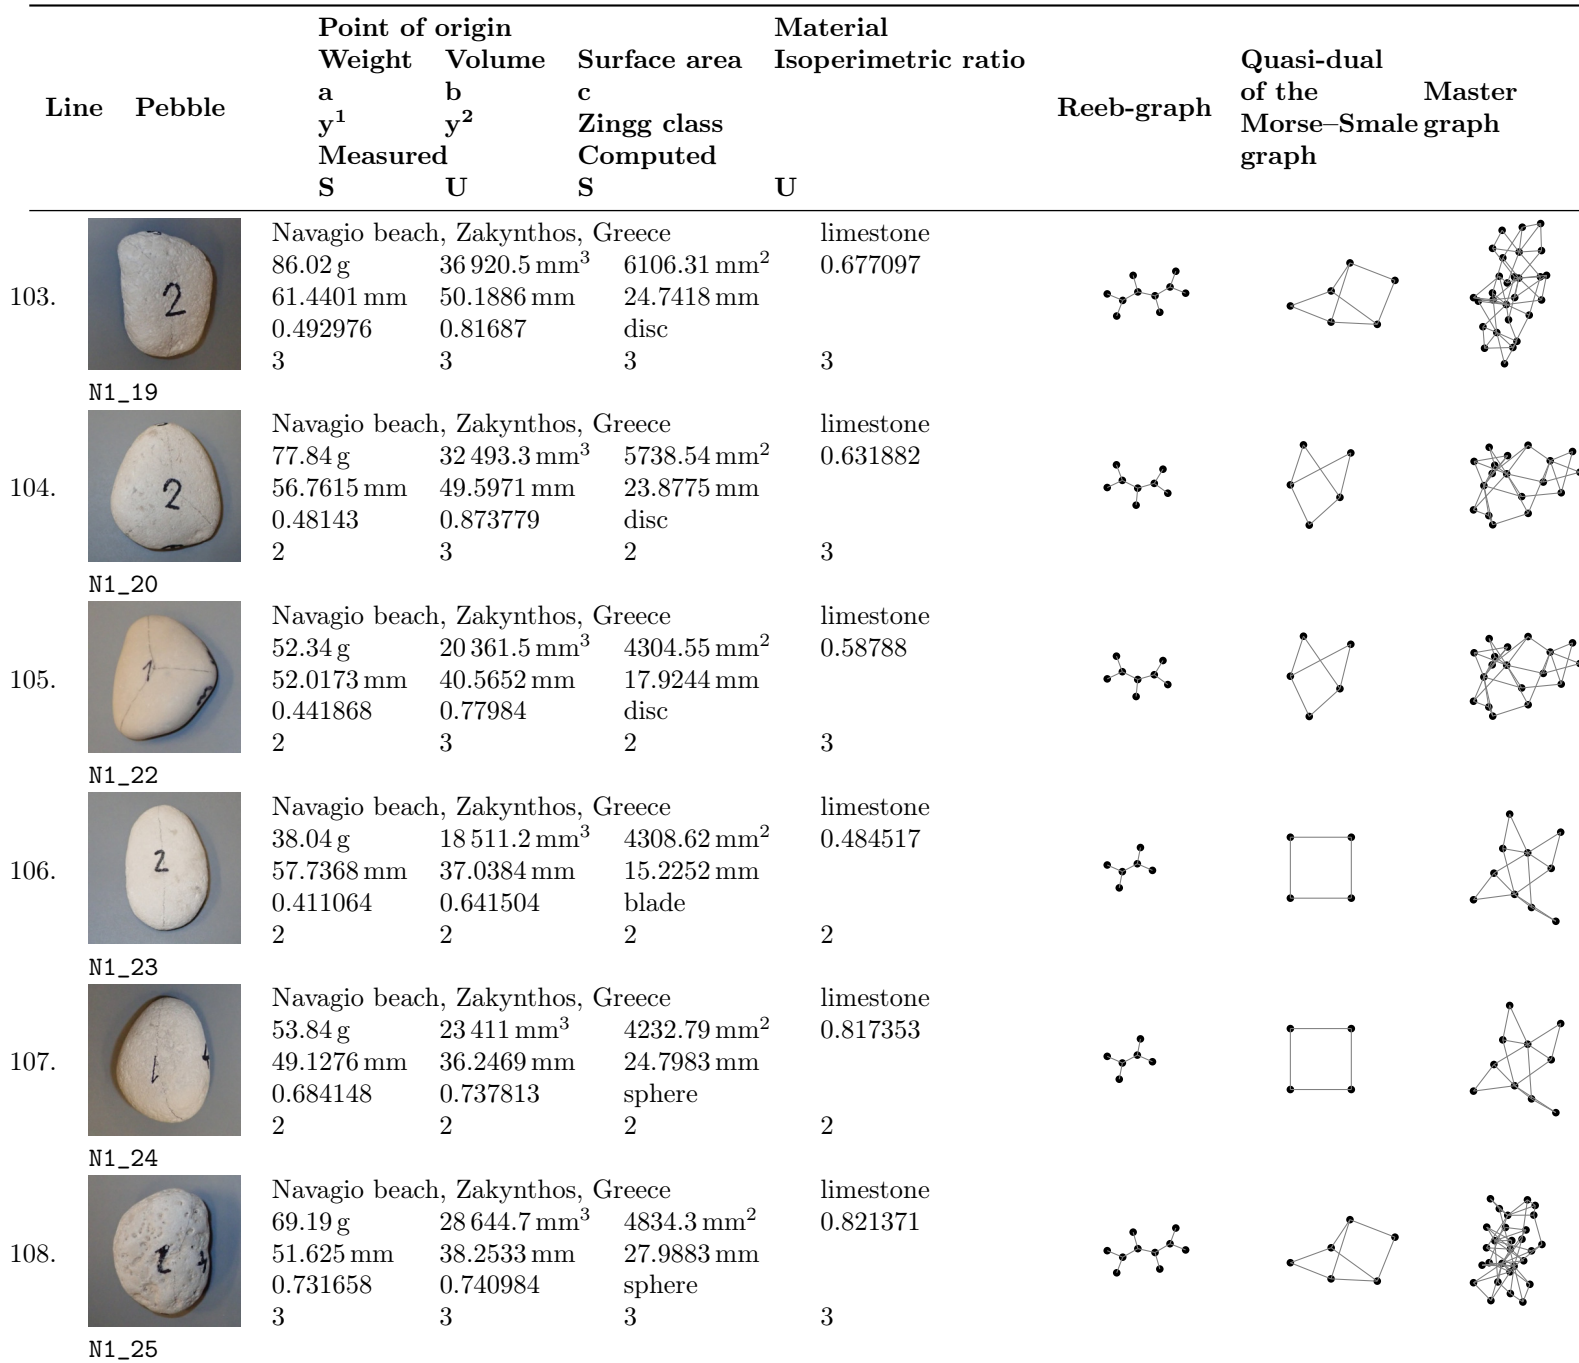   | 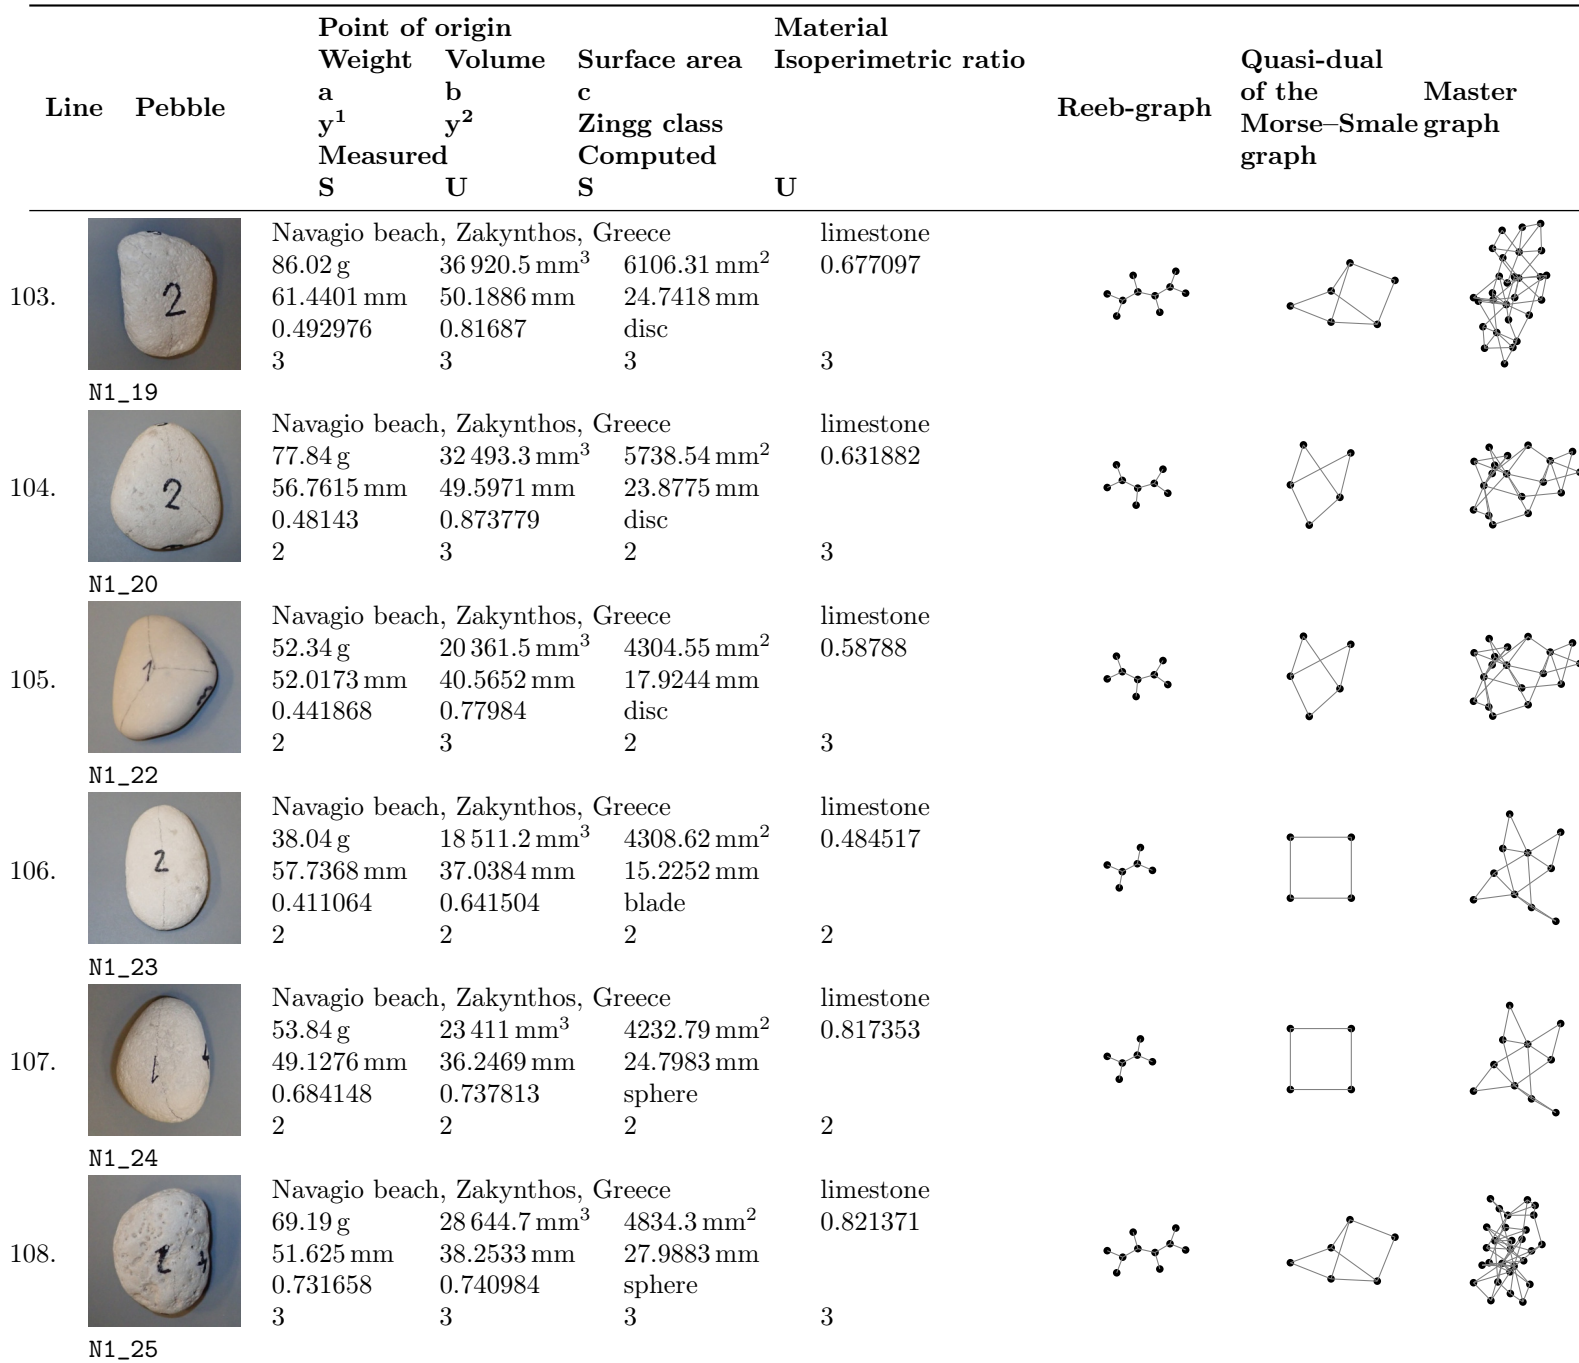   | 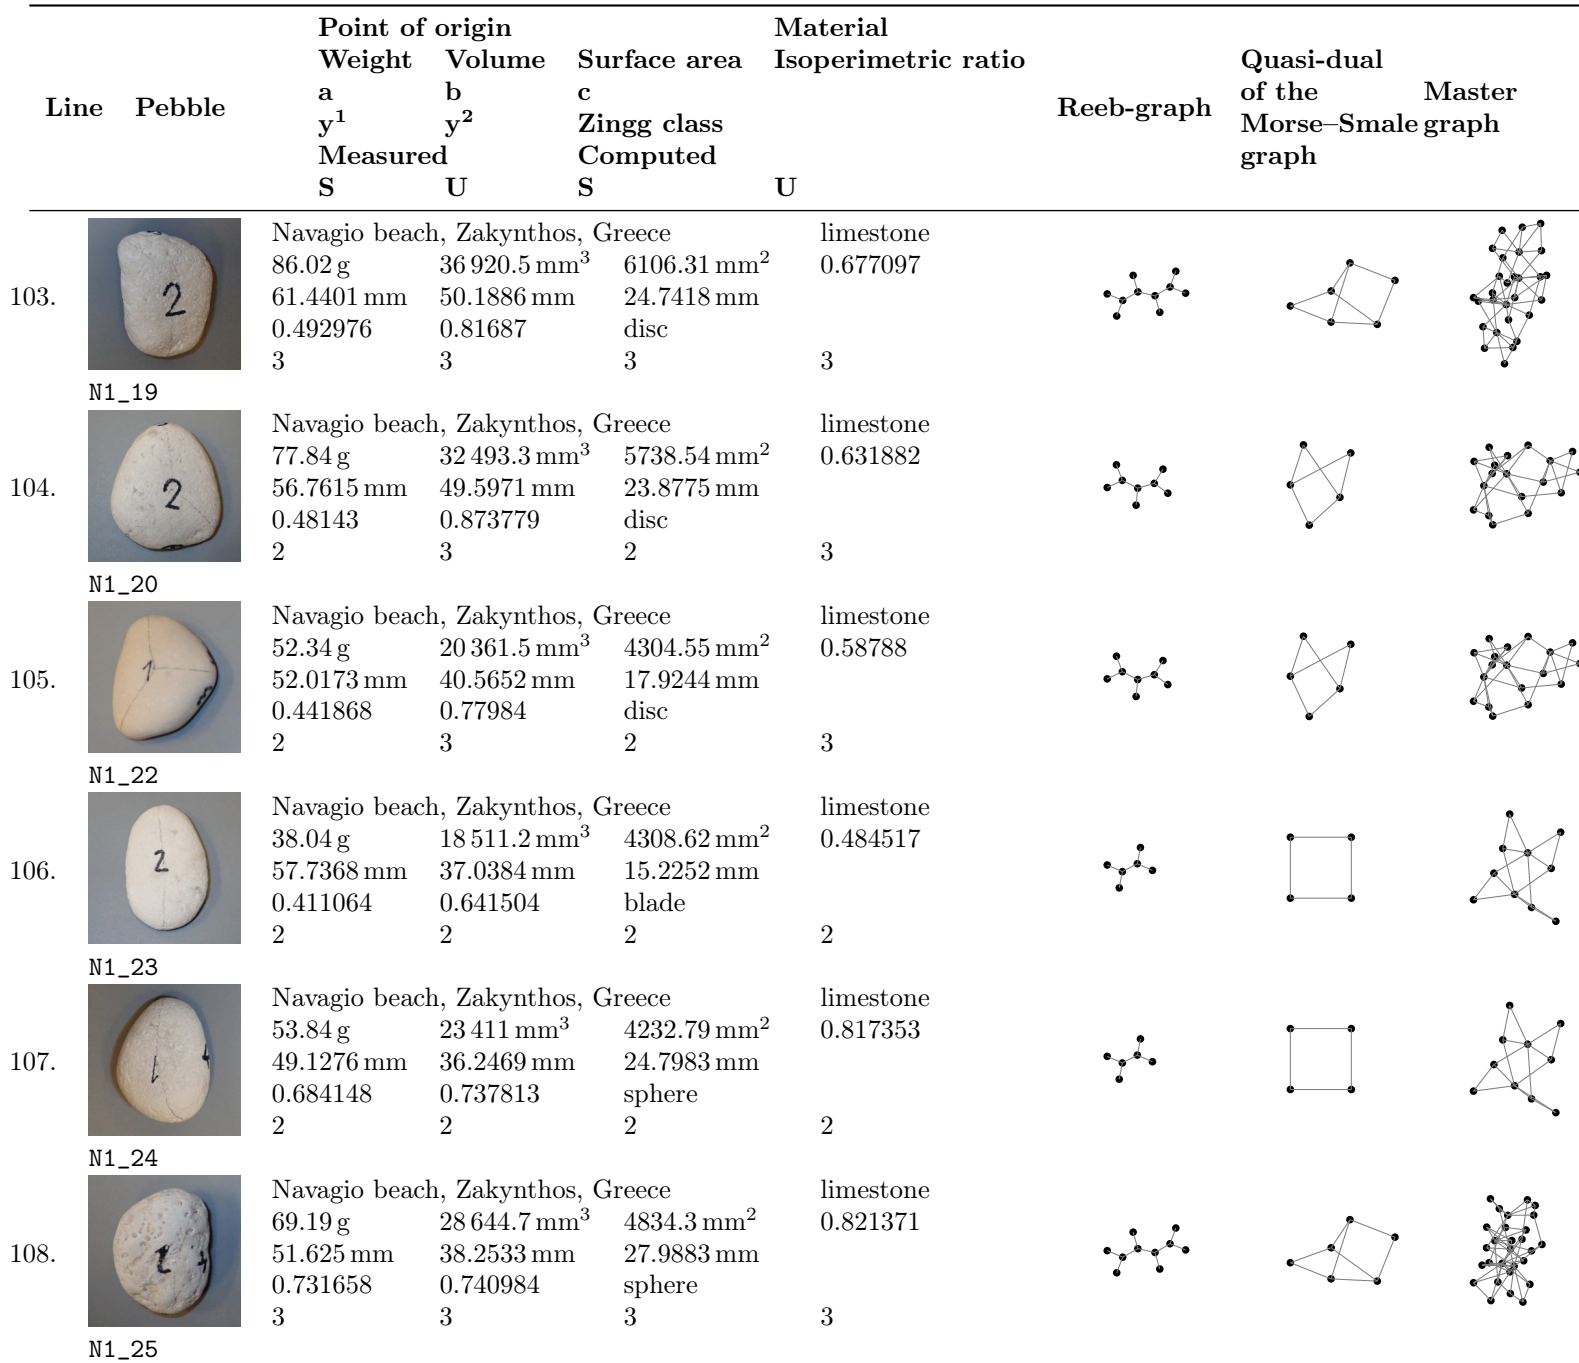   |
|      |                                                                                     | 86.02 g                          | 36 920.5 mm <sup>3</sup> | 6106.31 mm <sup>2</sup>      |           |                     |                                                                                       |                                                                                       |                                                                                       |
|      |                                                                                     | 61.4401 mm                       | 50.1886 mm               | 24.7418 mm                   |           |                     |                                                                                       |                                                                                       |                                                                                       |
|      |                                                                                     | 0.492976                         | 0.81687                  | disc                         |           |                     |                                                                                       |                                                                                       |                                                                                       |
|      | N1_19                                                                               | 3                                | 3                        | 3                            | 3         |                     |                                                                                       |                                                                                       |                                                                                       |
| 104. | 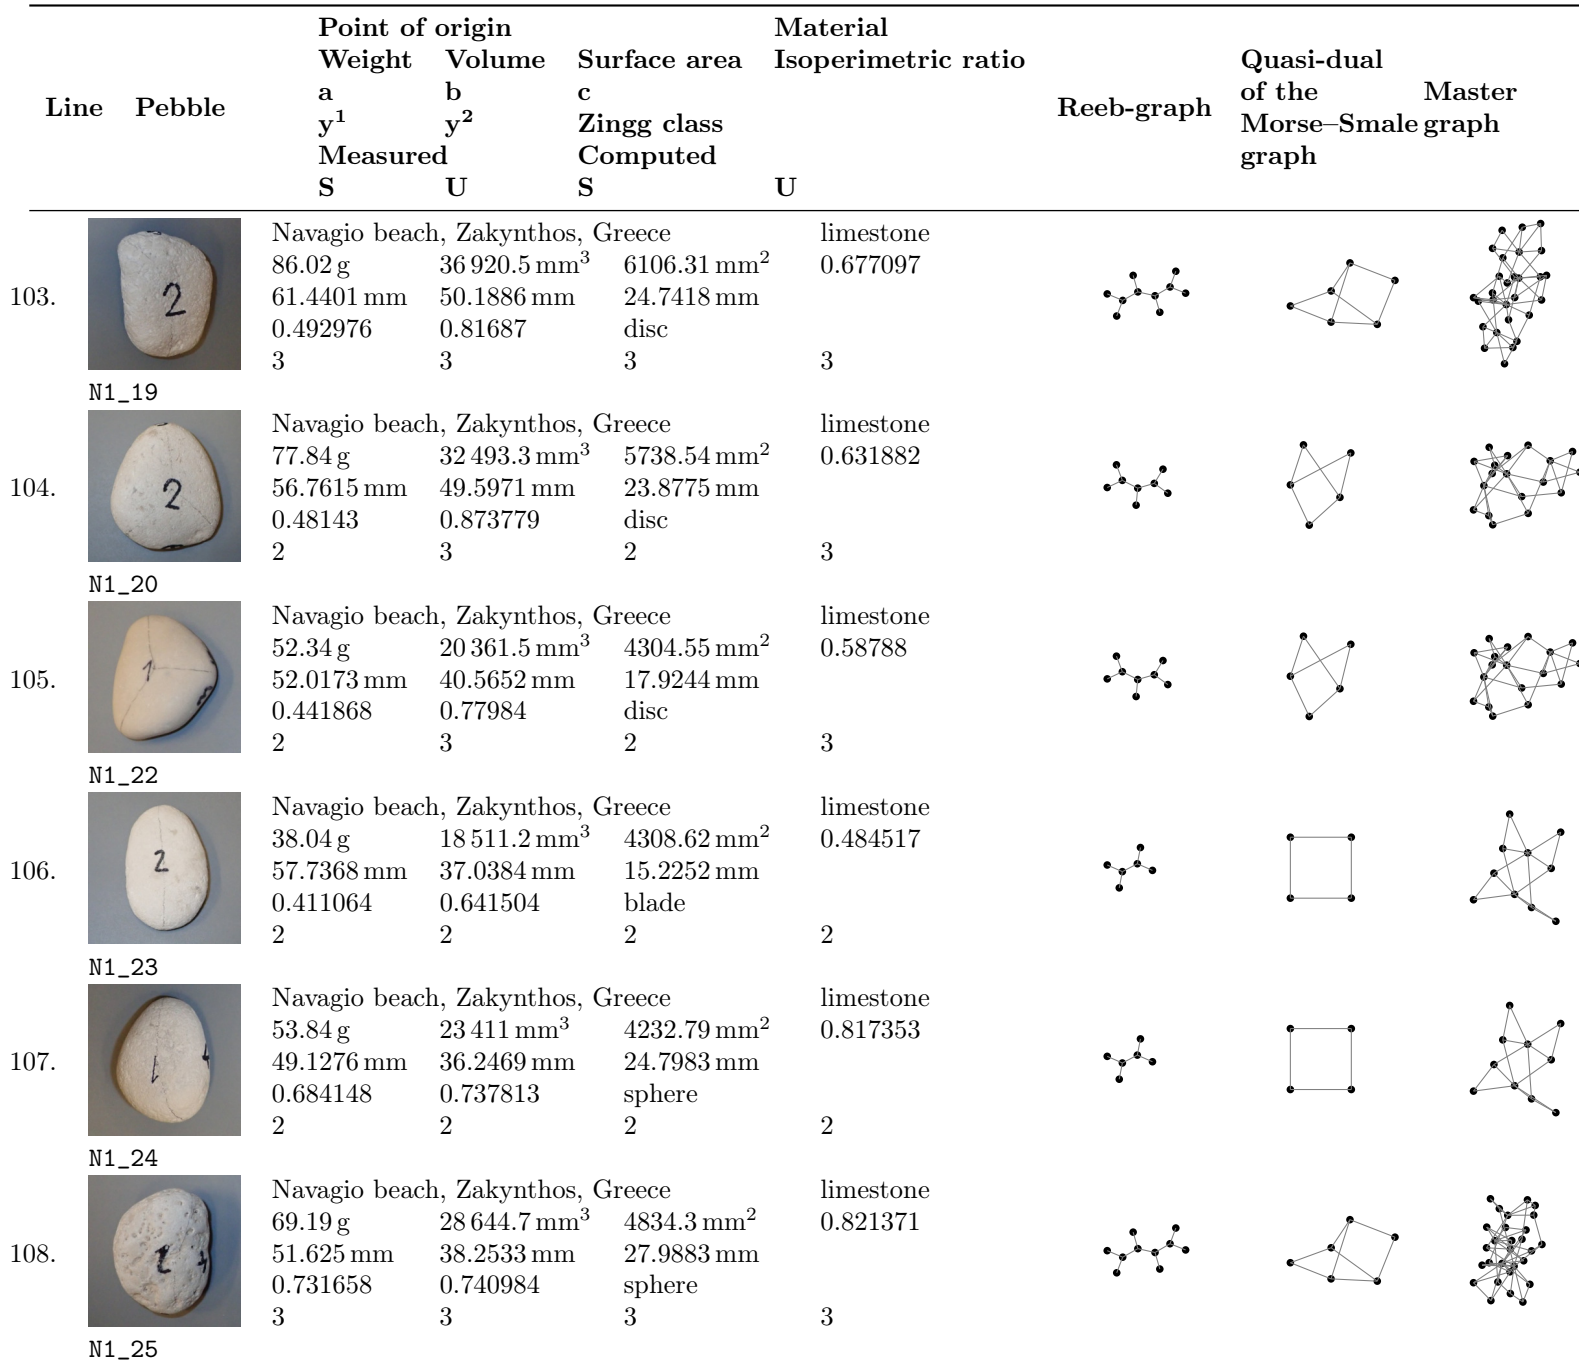   | Navagio beach, Zakynthos, Greece |                          |                              | limestone | 0.631882            | 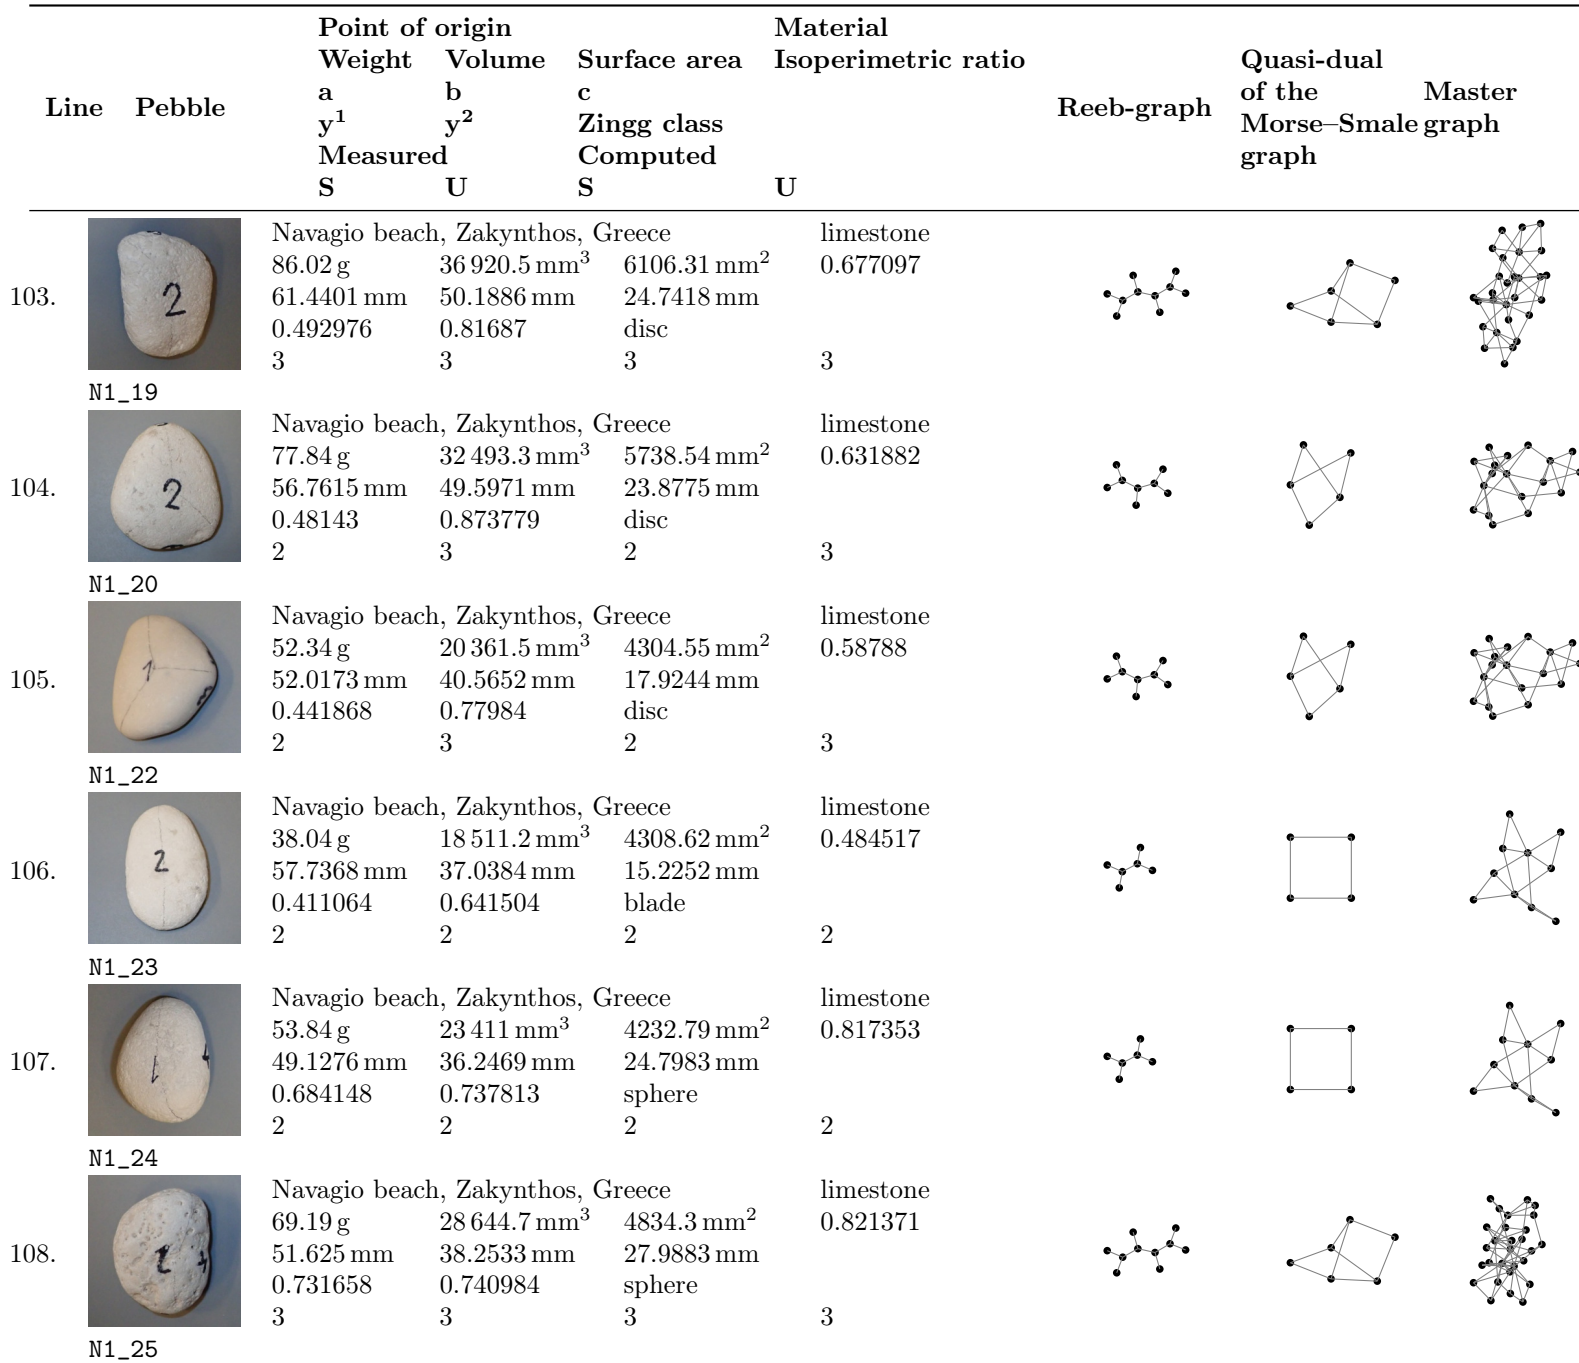   | 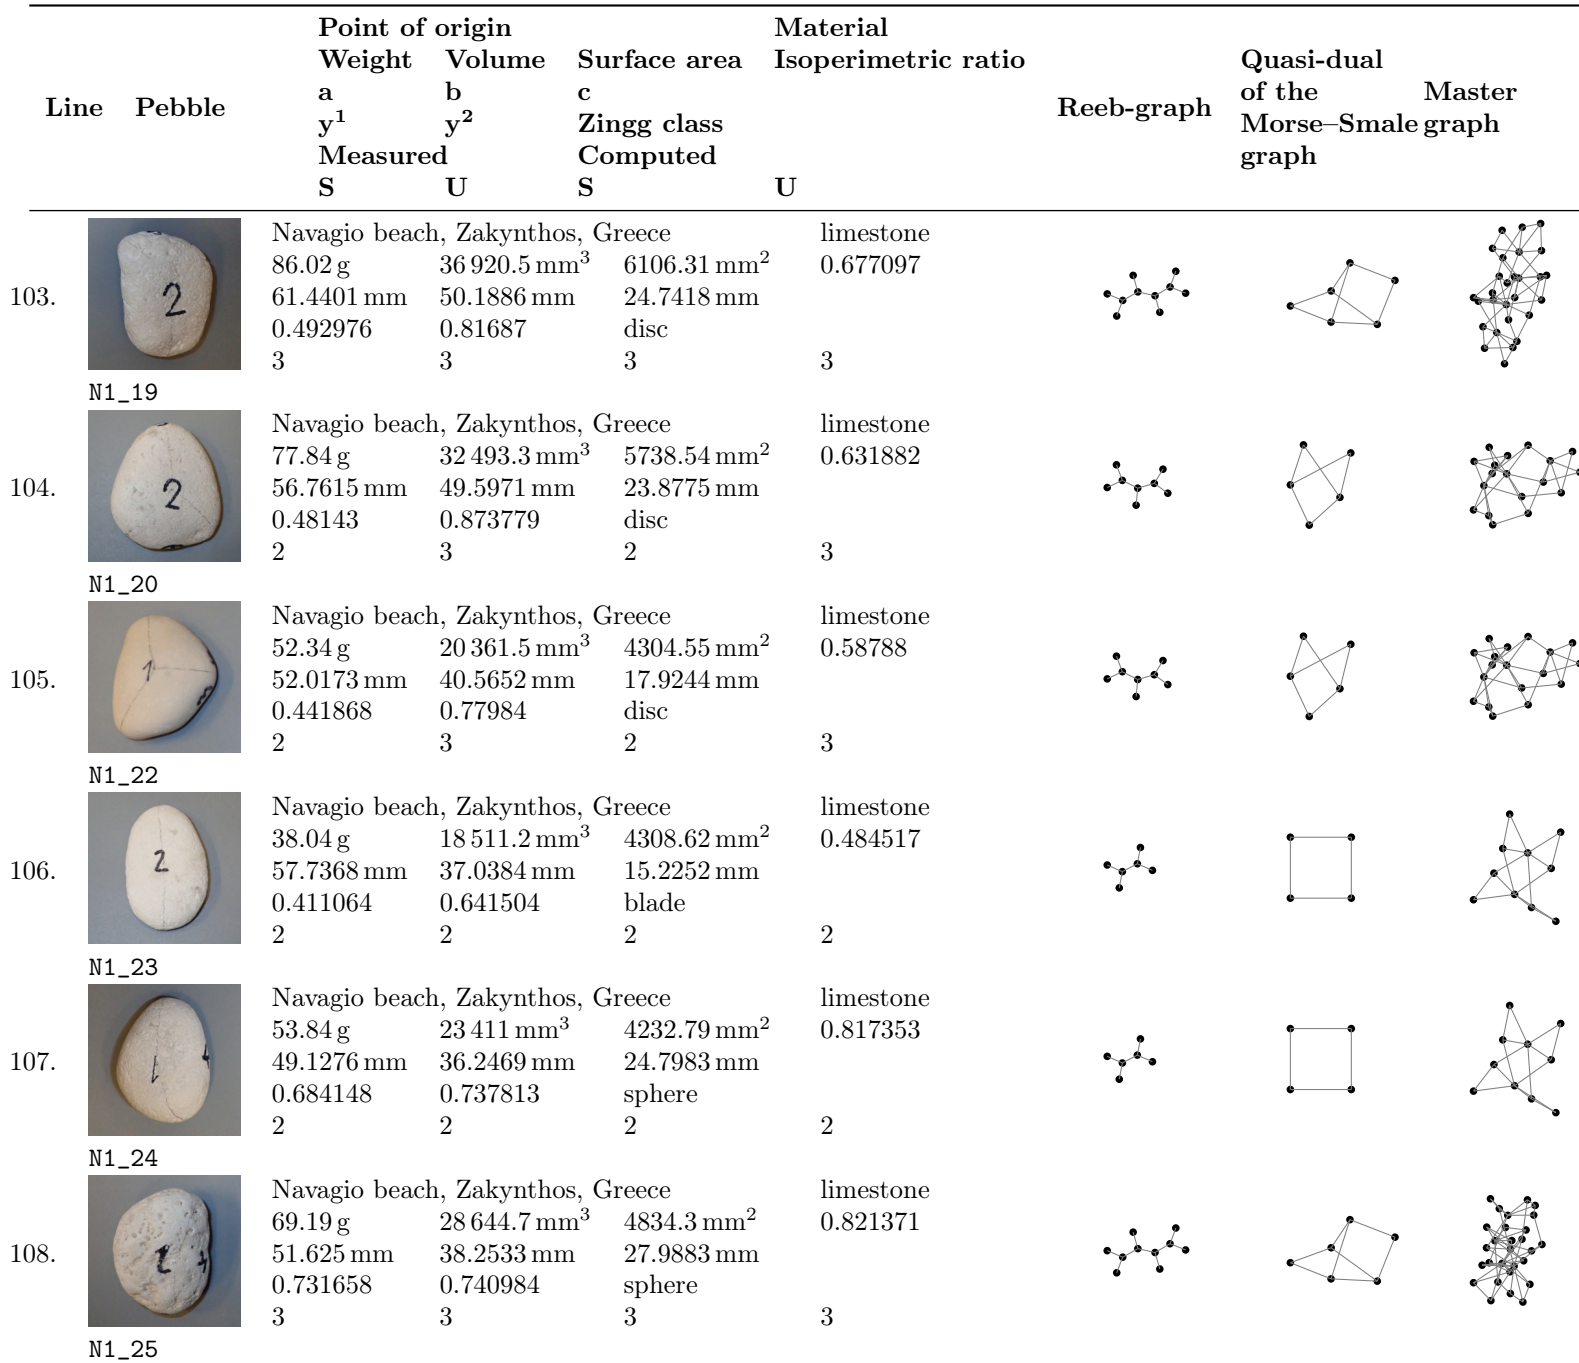   | 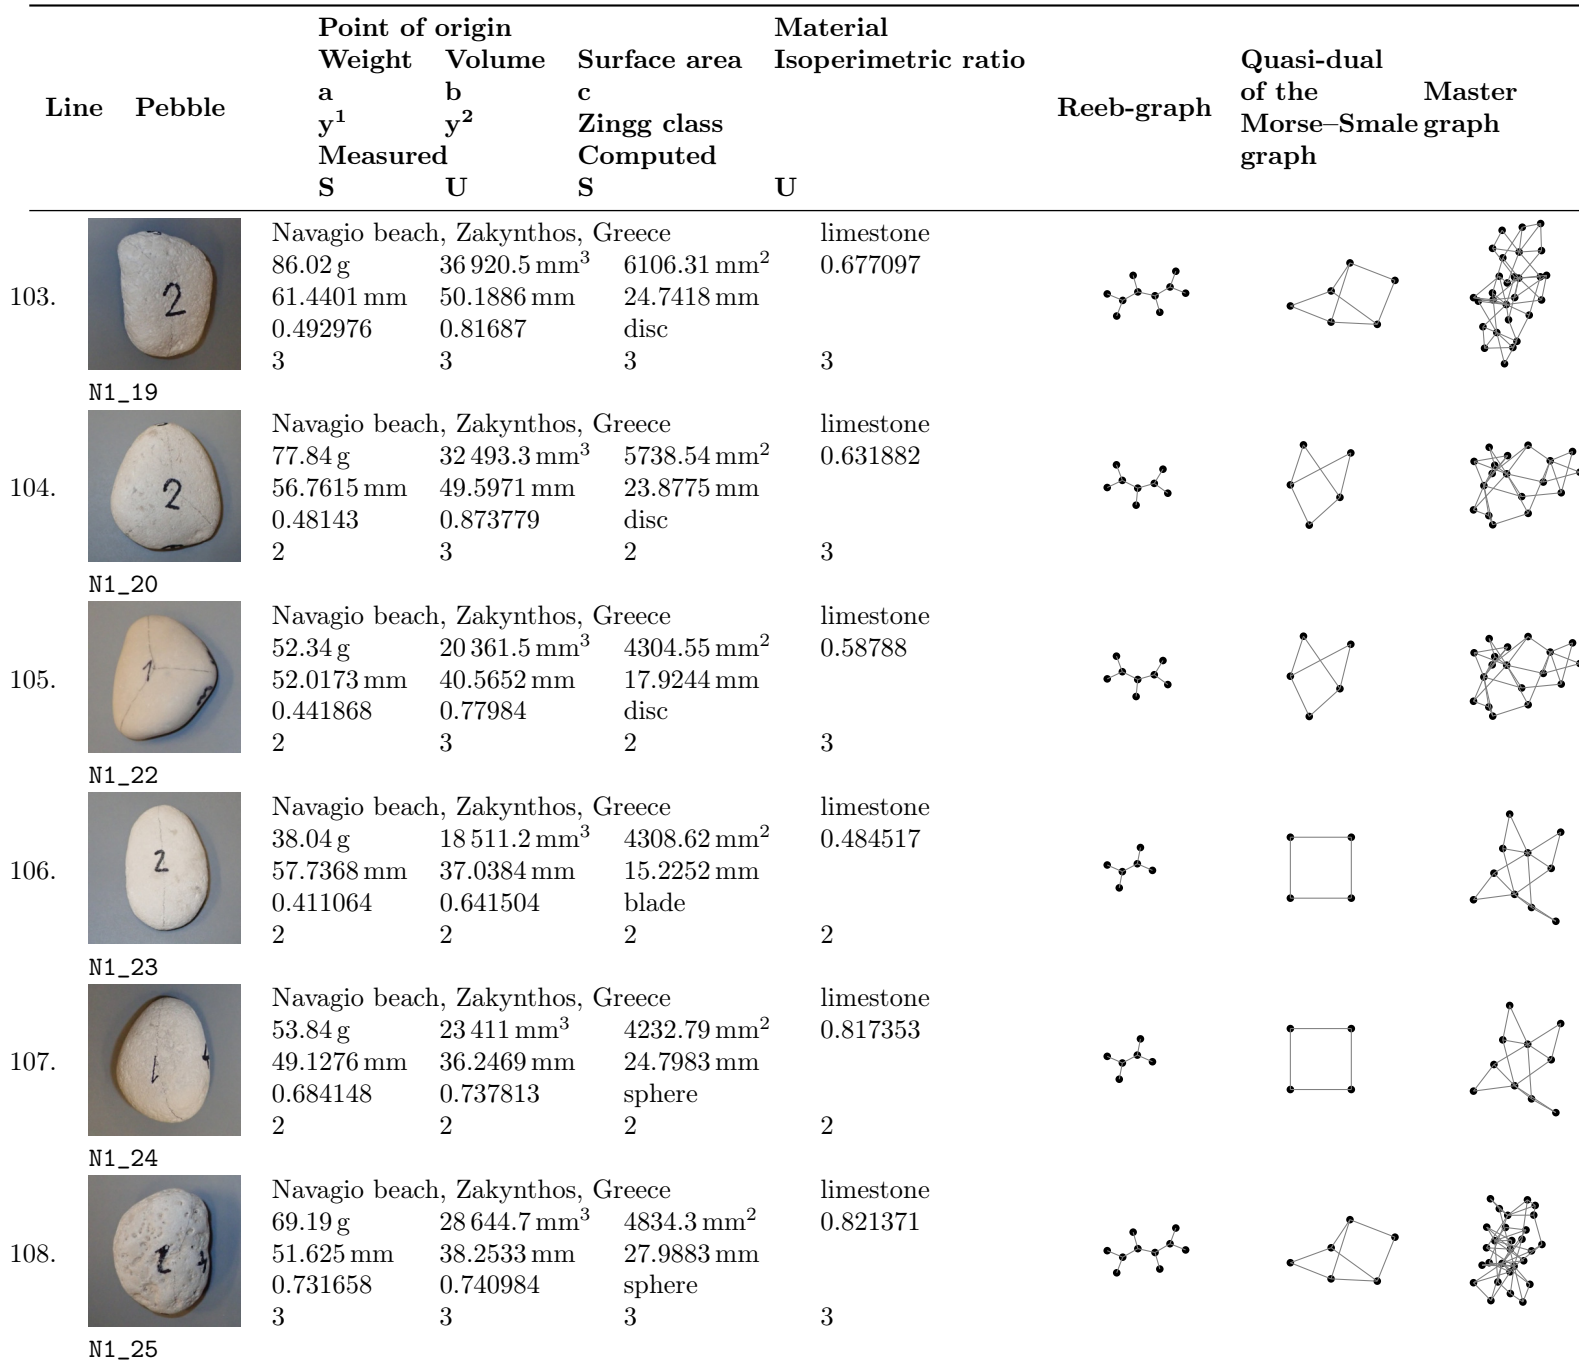   |
|      |                                                                                     | 77.84 g                          | 32 493.3 mm <sup>3</sup> | 5738.54 mm <sup>2</sup>      |           |                     |                                                                                       |                                                                                       |                                                                                       |
|      |                                                                                     | 56.7615 mm                       | 49.5971 mm               | 23.8775 mm                   |           |                     |                                                                                       |                                                                                       |                                                                                       |
|      |                                                                                     | 0.48143                          | 0.873779                 | disc                         |           |                     |                                                                                       |                                                                                       |                                                                                       |
|      | N1_20                                                                               | 2                                | 3                        | 2                            | 3         |                     |                                                                                       |                                                                                       |                                                                                       |
| 105. | 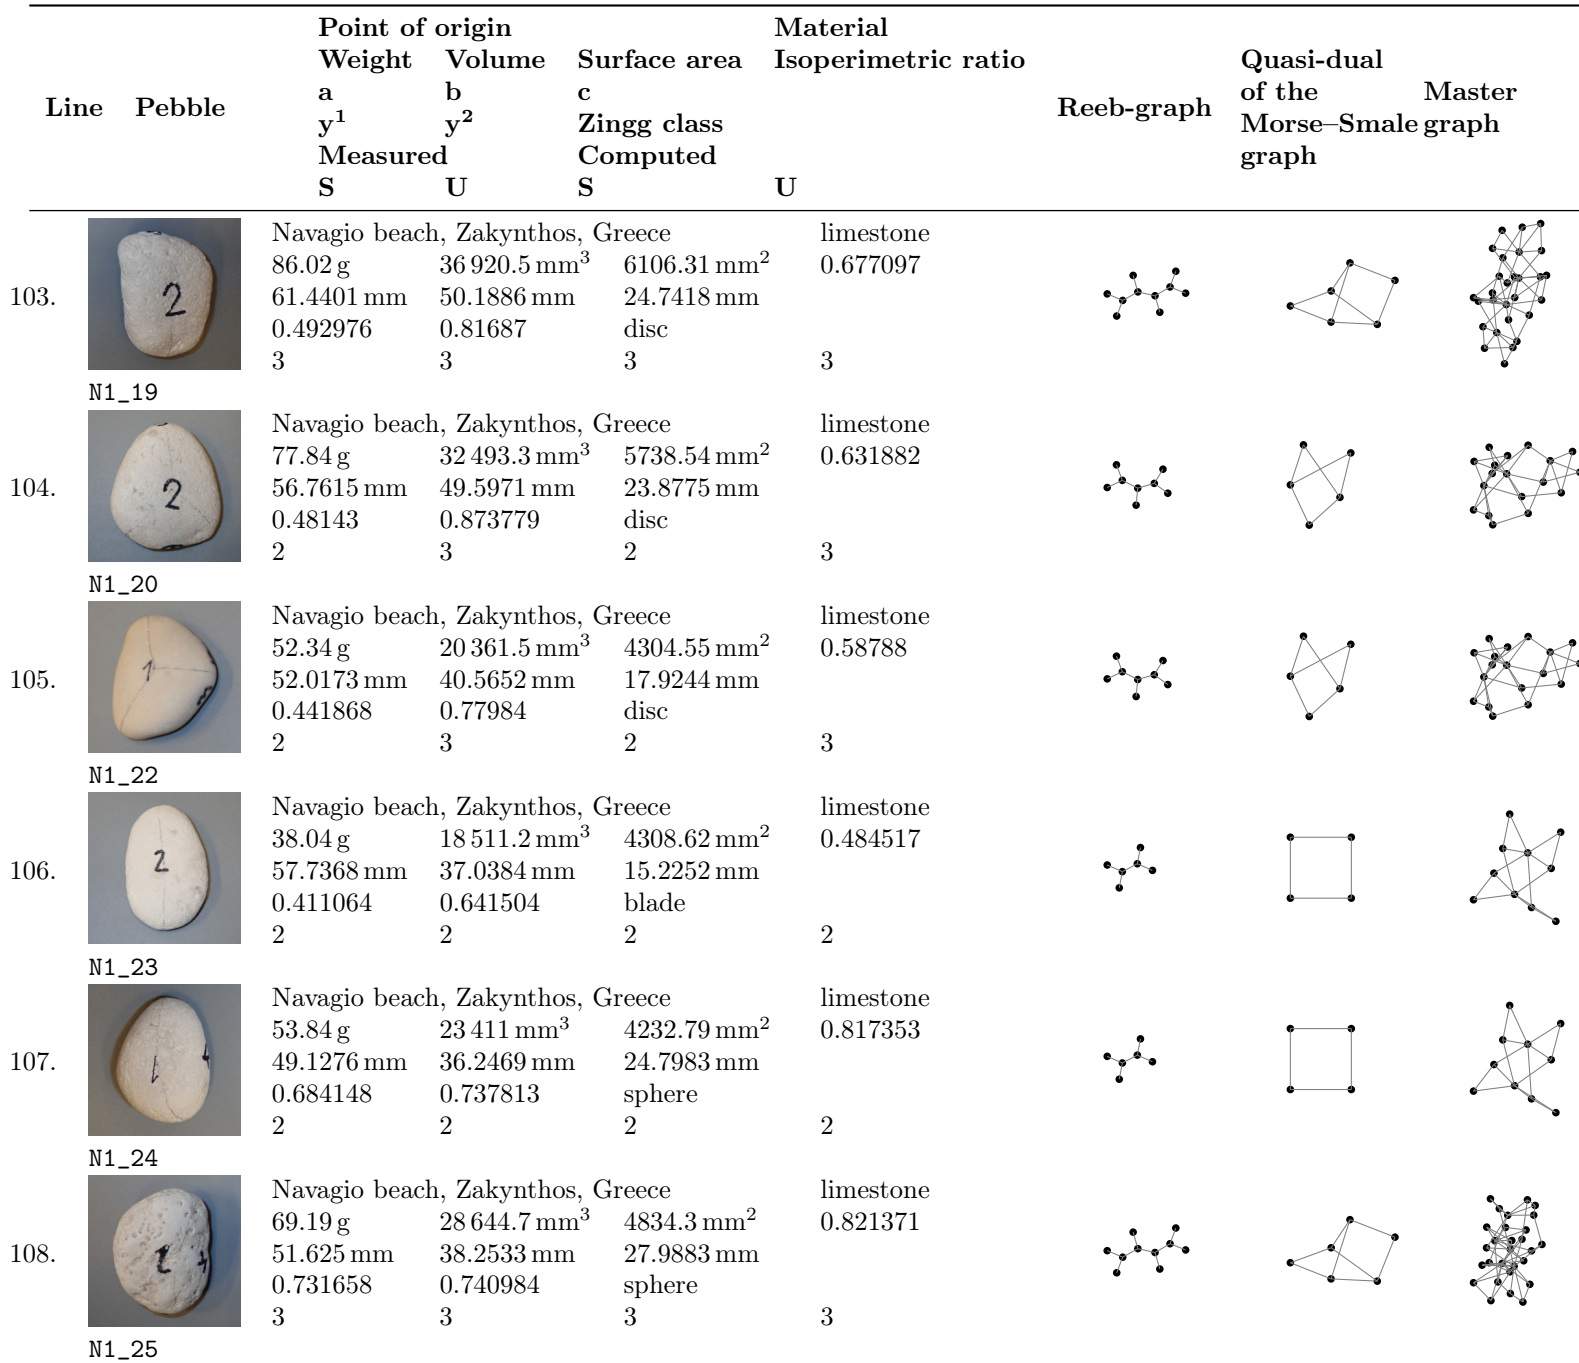   | Navagio beach, Zakynthos, Greece |                          |                              | limestone | 0.58788             | 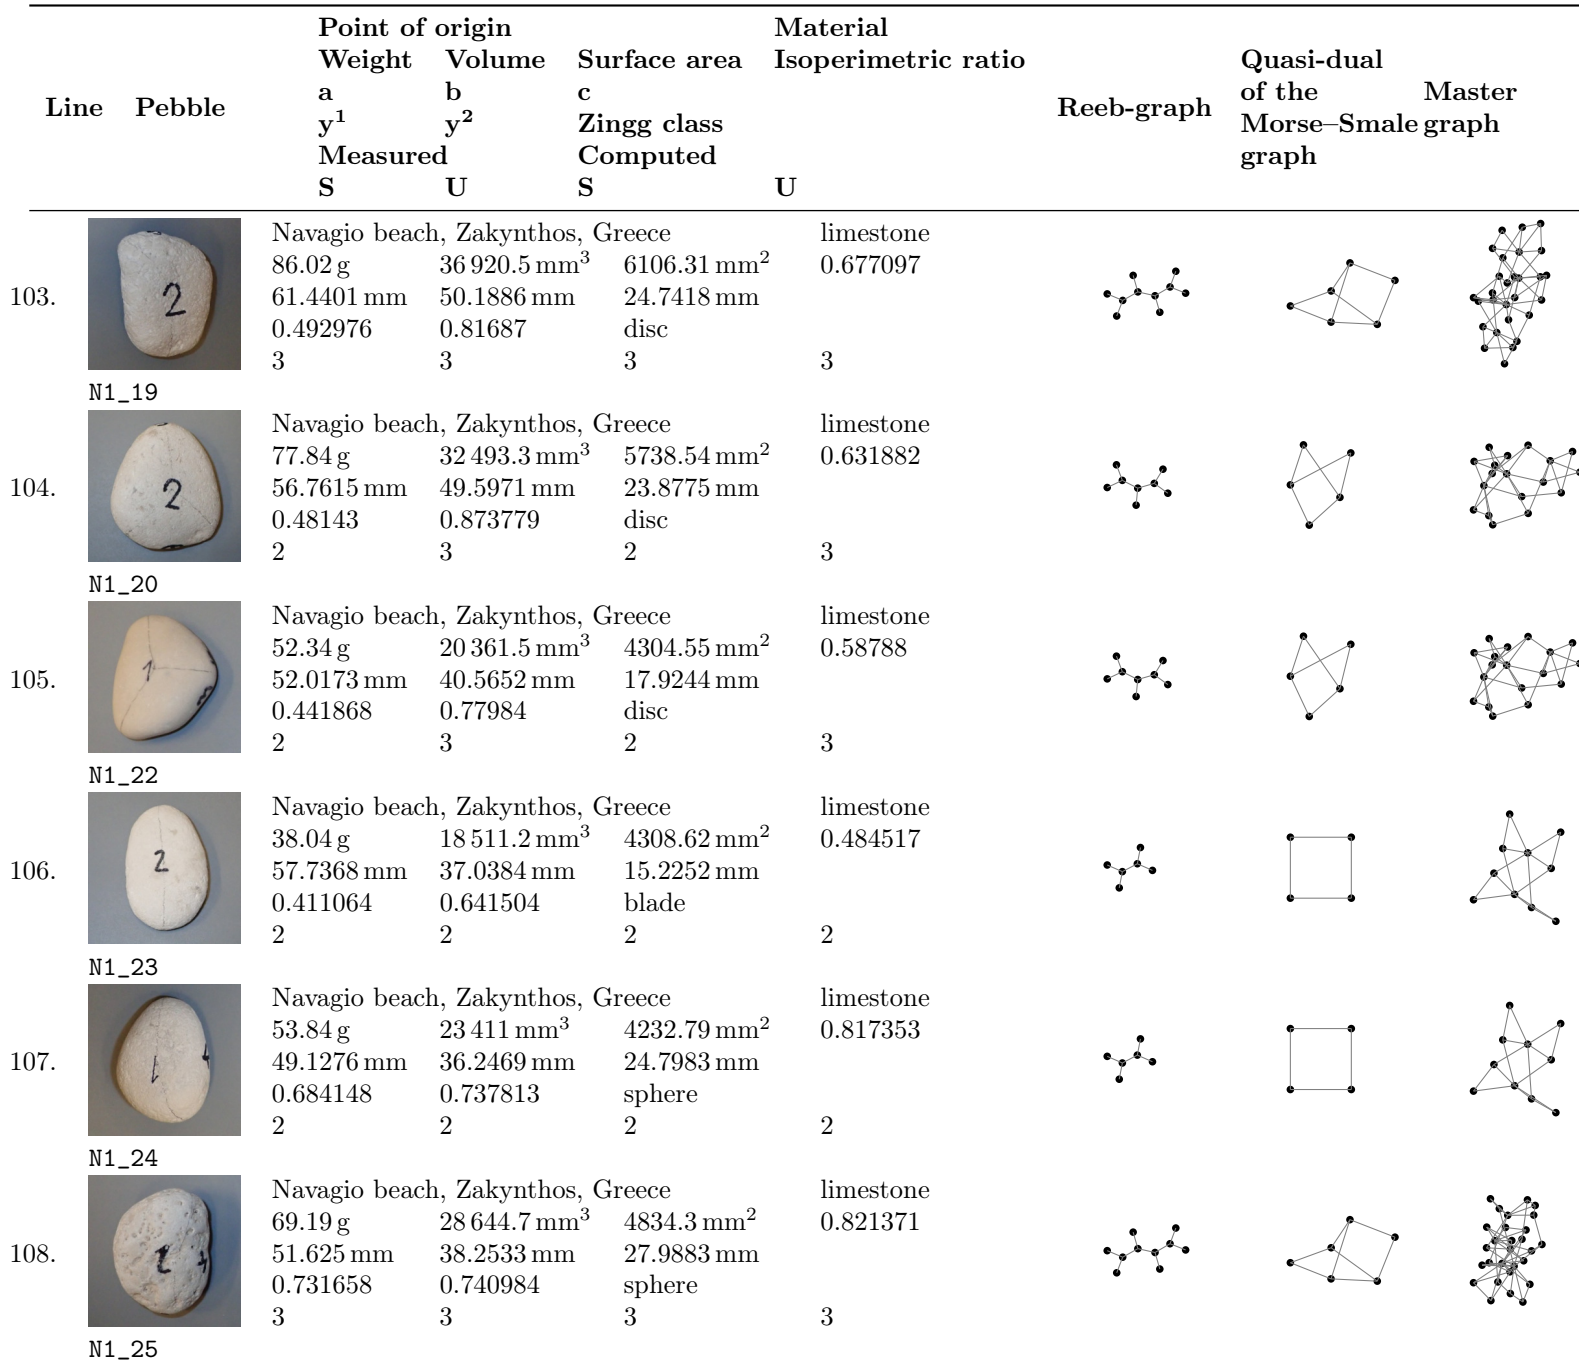   | 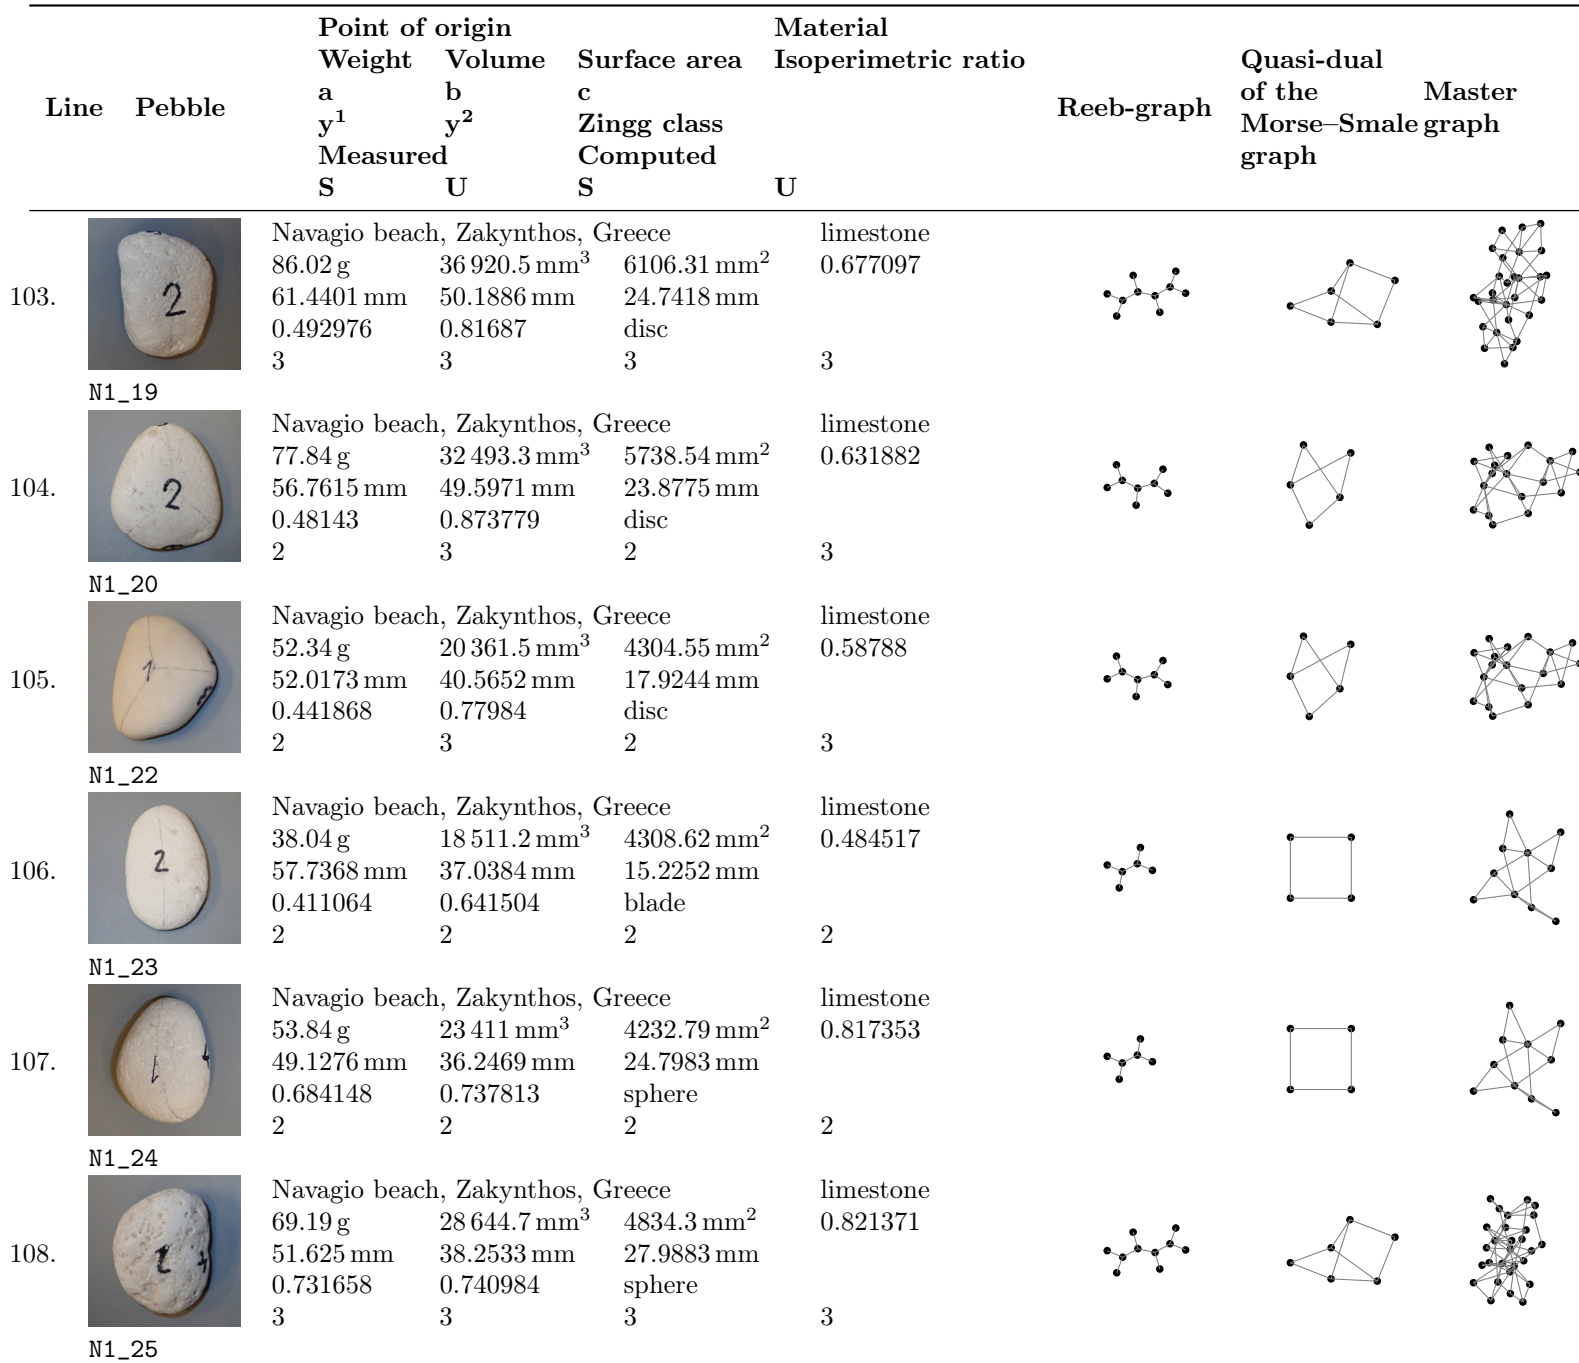   | 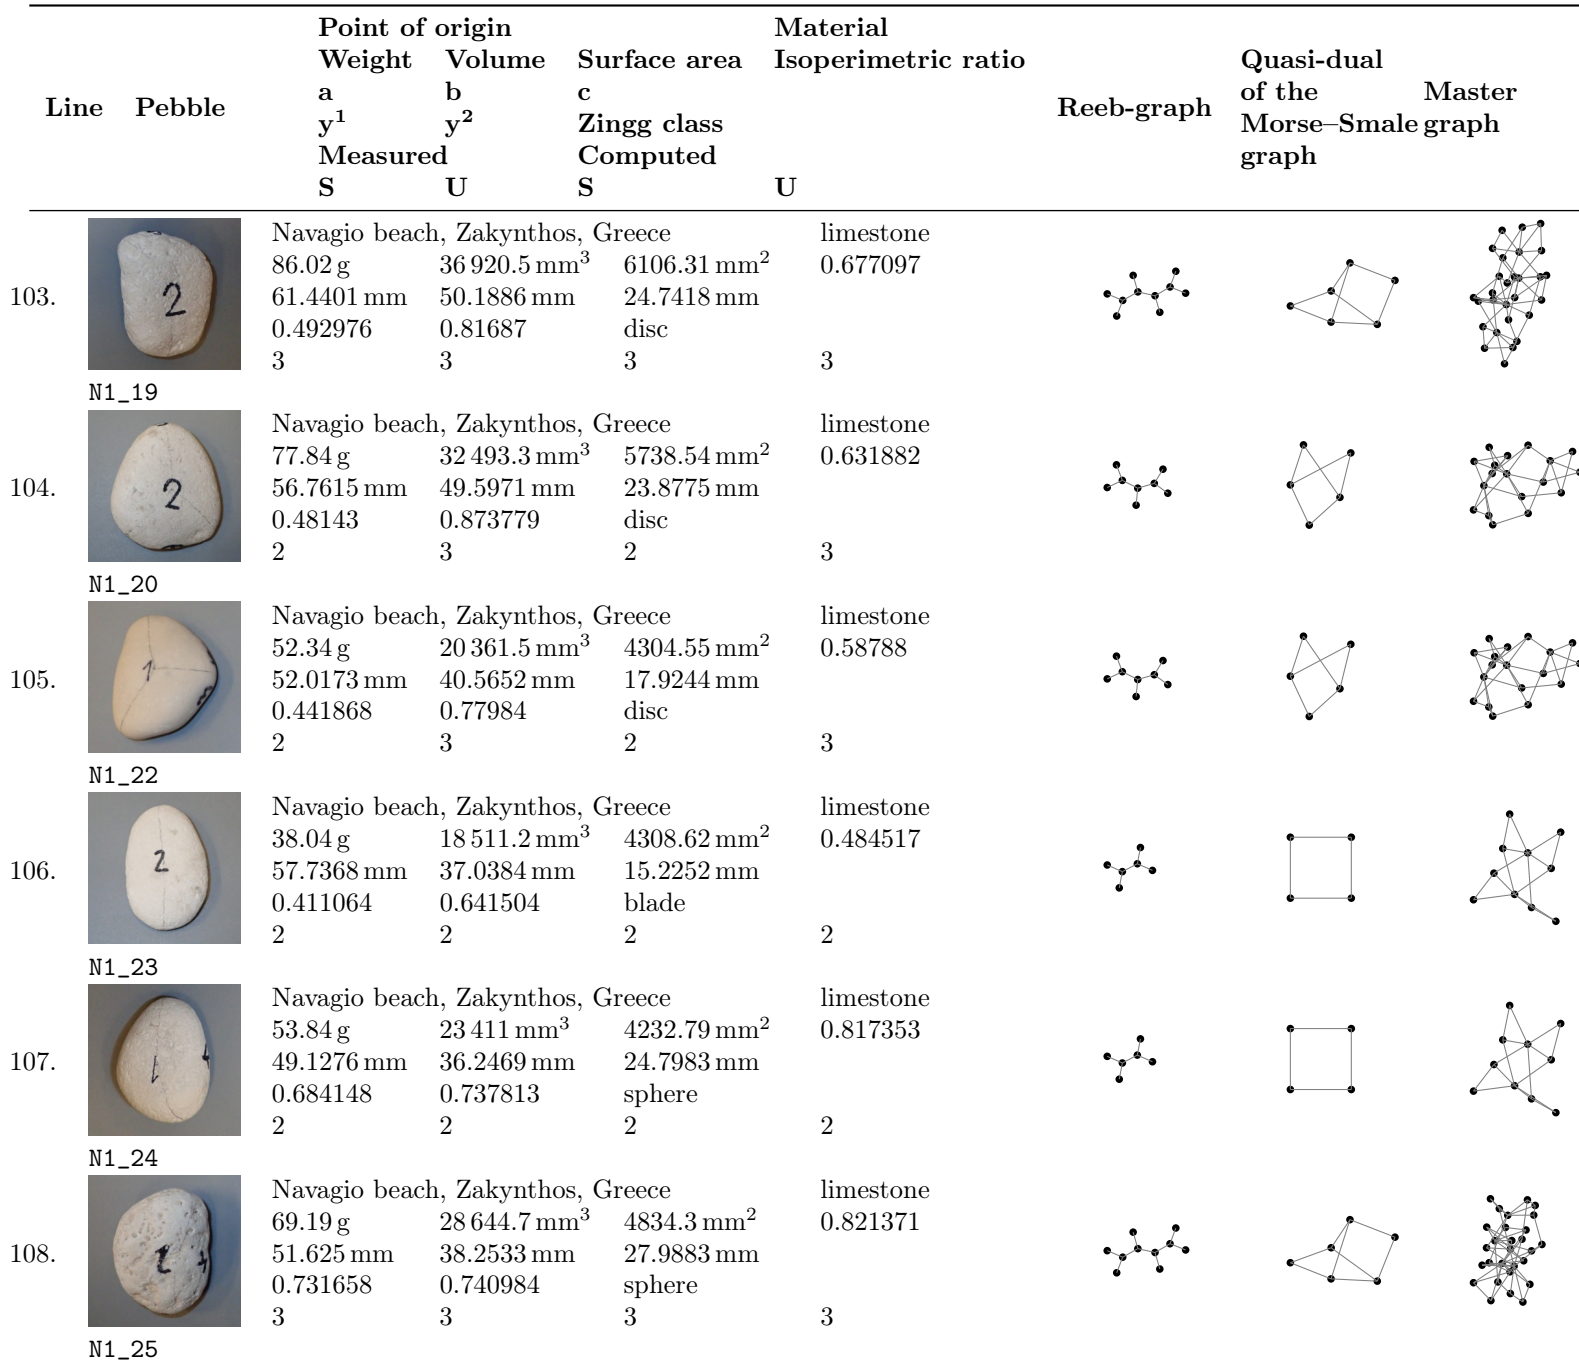   |
|      |                                                                                     | 52.34 g                          | 20 361.5 mm <sup>3</sup> | 4304.55 mm <sup>2</sup>      |           |                     |                                                                                       |                                                                                       |                                                                                       |
|      |                                                                                     | 52.0173 mm                       | 40.5652 mm               | 17.9244 mm                   |           |                     |                                                                                       |                                                                                       |                                                                                       |
|      |                                                                                     | 0.441868                         | 0.77984                  | disc                         |           |                     |                                                                                       |                                                                                       |                                                                                       |
|      | N1_22                                                                               | 2                                | 3                        | 2                            | 3         |                     |                                                                                       |                                                                                       |                                                                                       |
| 106. | 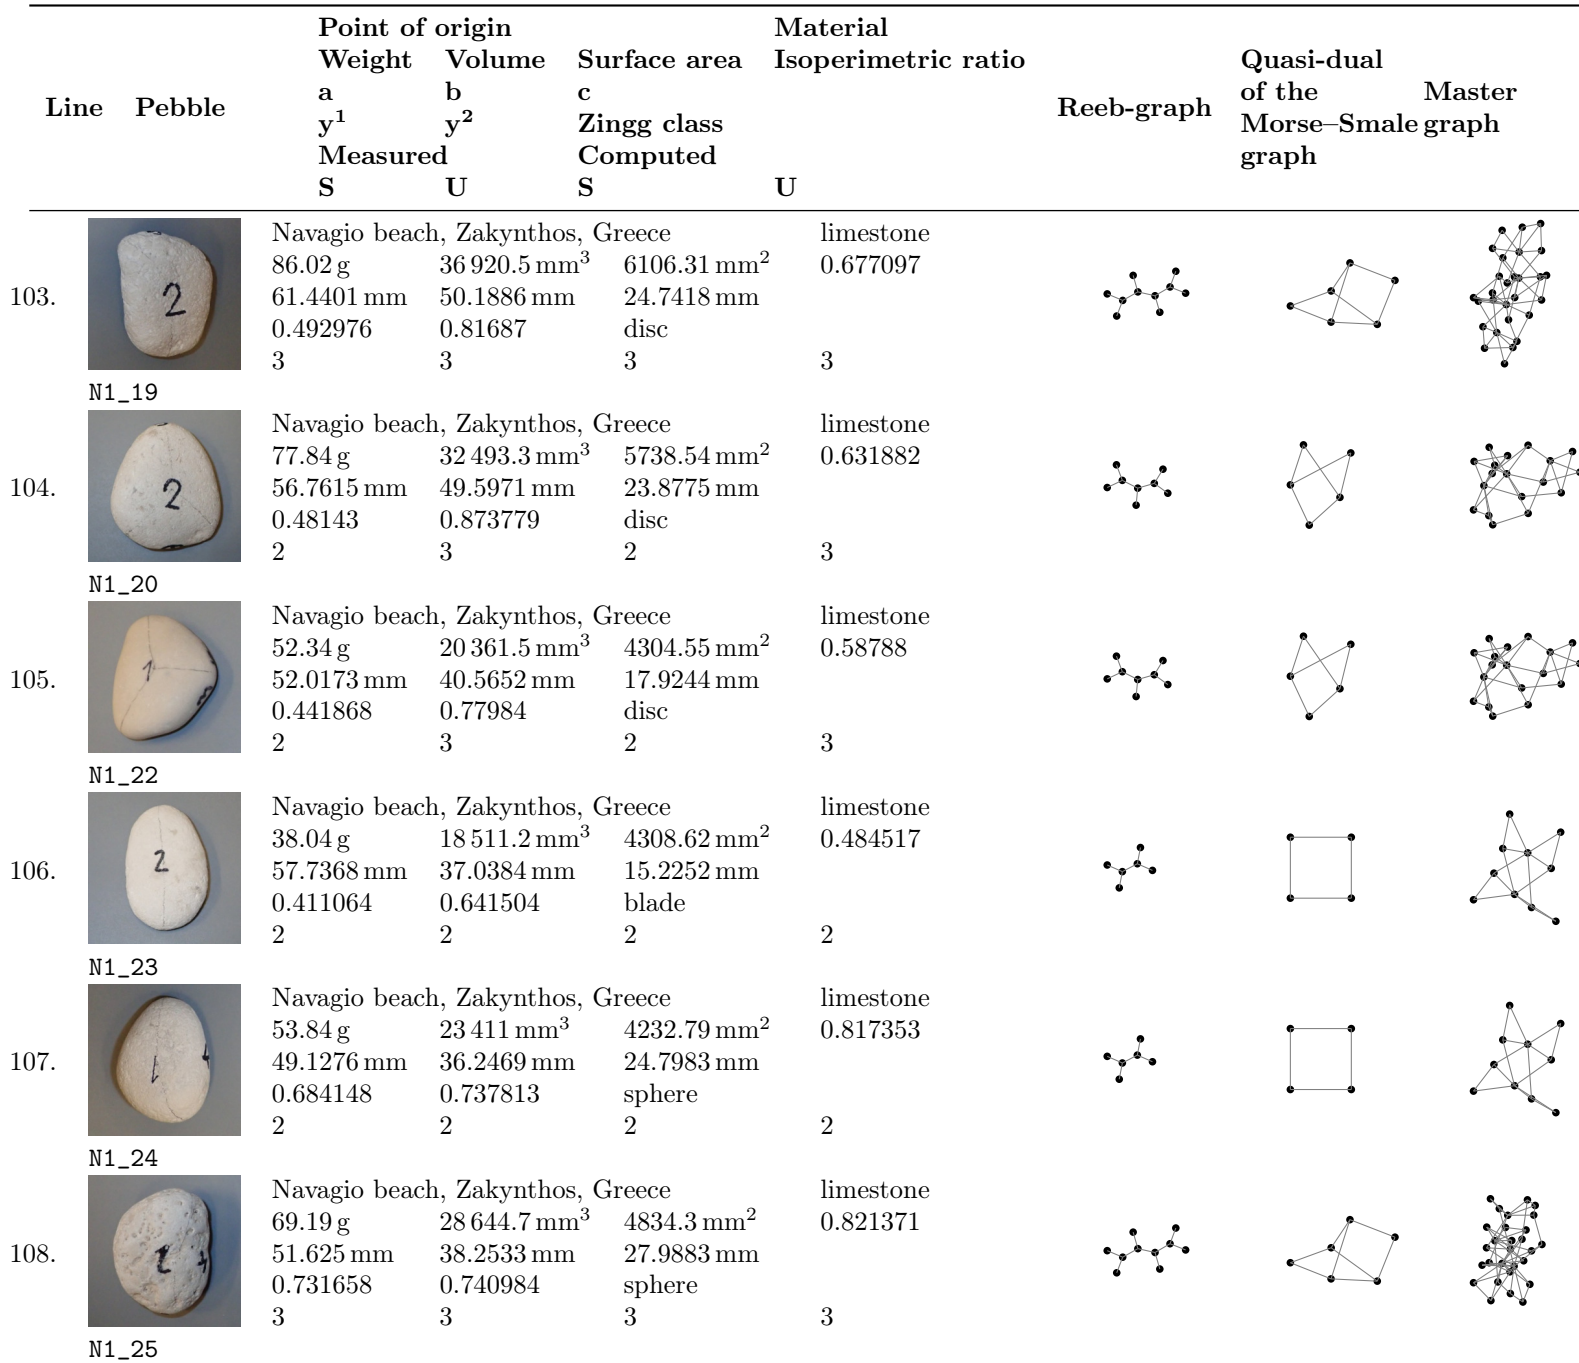  | Navagio beach, Zakynthos, Greece |                          |                              | limestone | 0.484517            | 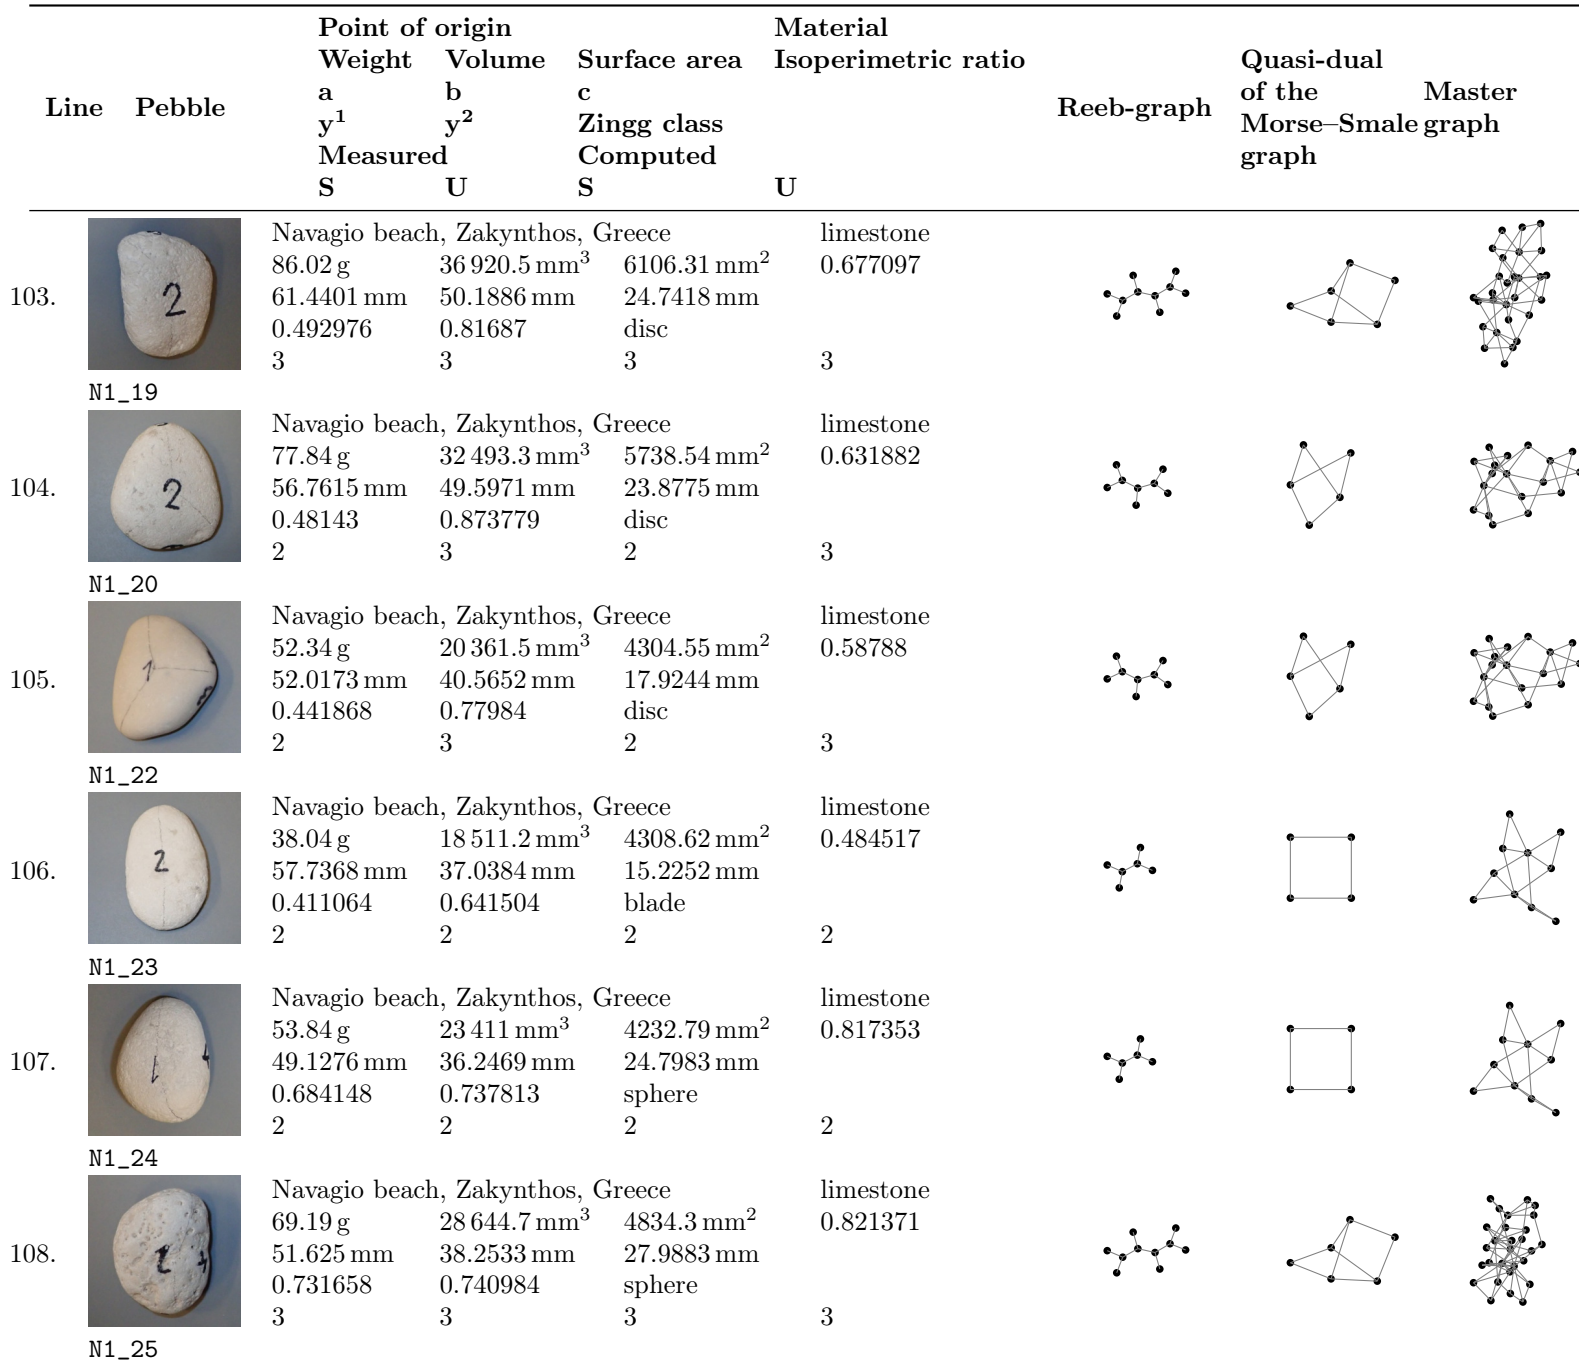  | 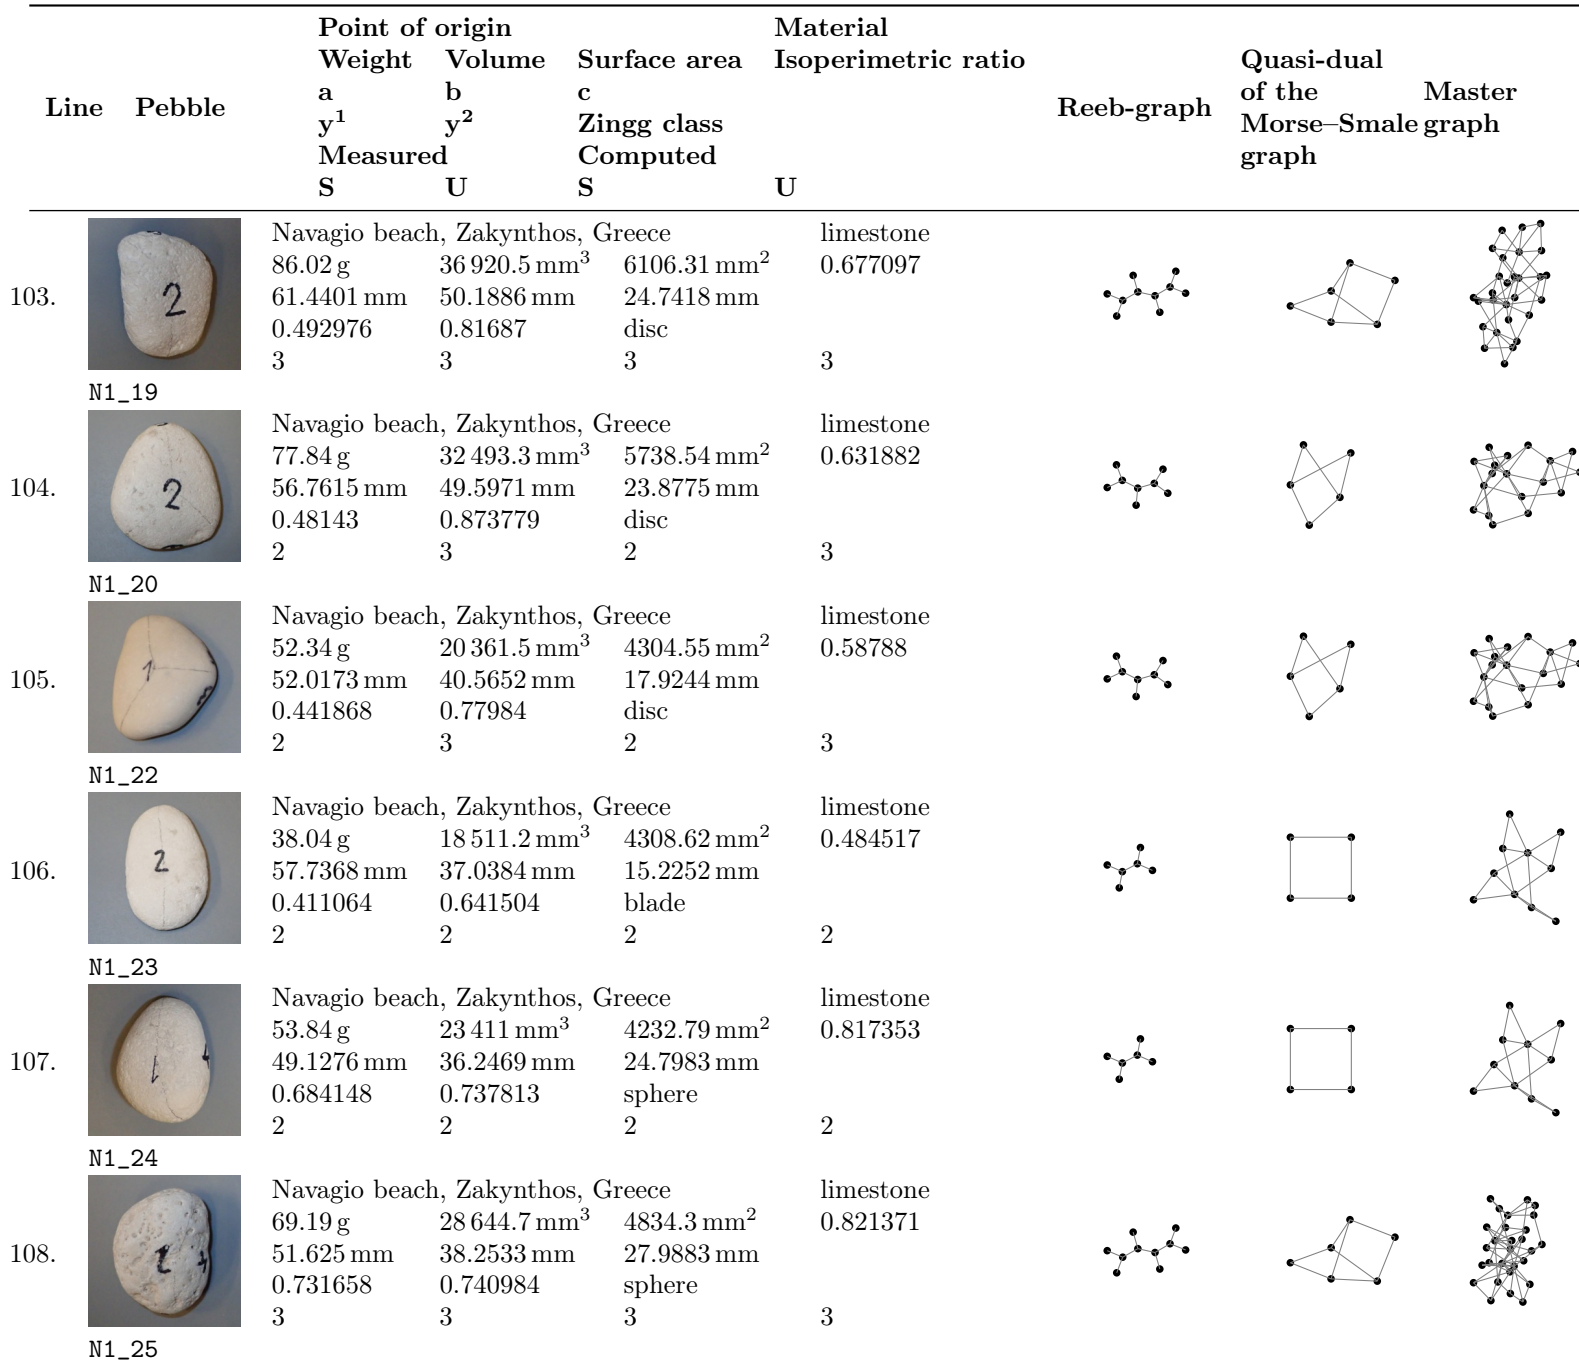  | 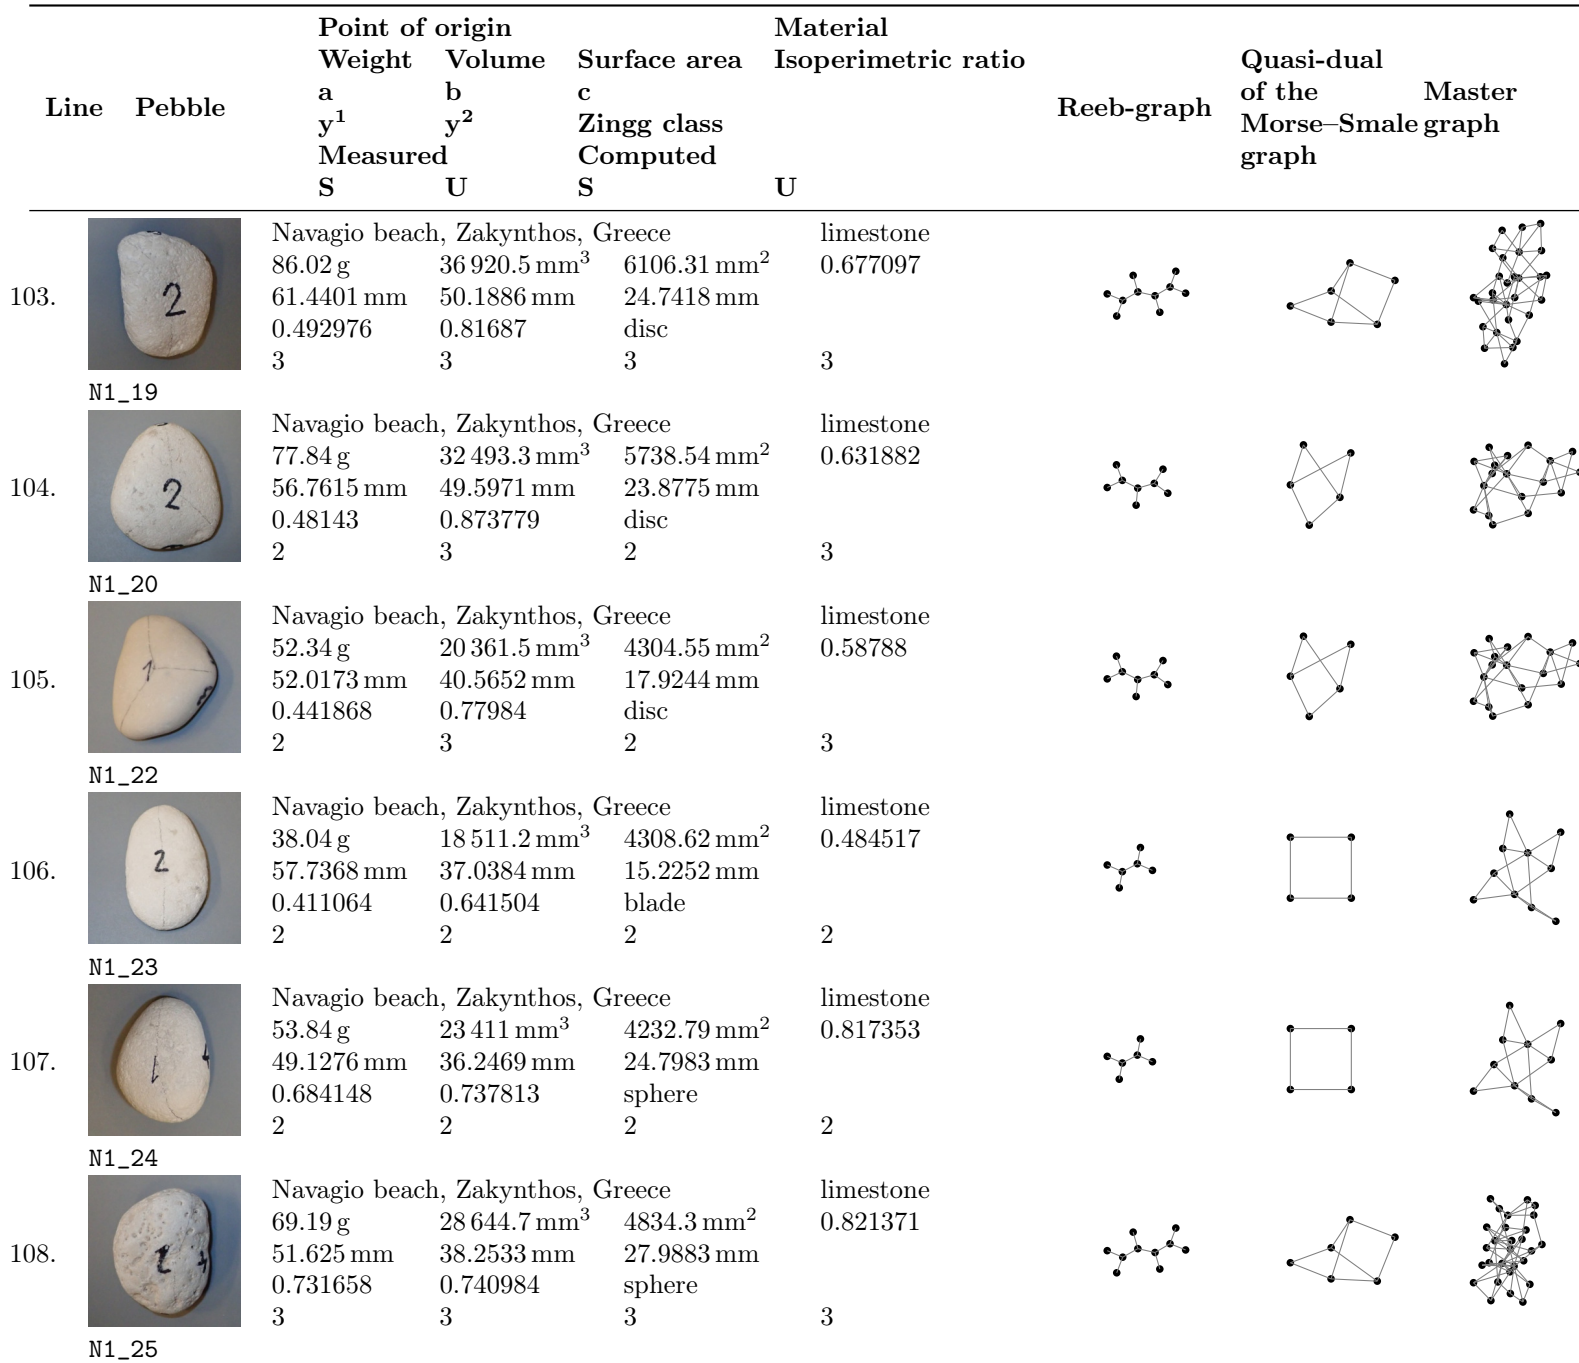  |
|      |                                                                                     | 38.04 g                          | 18 511.2 mm <sup>3</sup> | 4308.62 mm <sup>2</sup>      |           |                     |                                                                                       |                                                                                       |                                                                                       |
|      |                                                                                     | 57.7368 mm                       | 37.0384 mm               | 15.2252 mm                   |           |                     |                                                                                       |                                                                                       |                                                                                       |
|      |                                                                                     | 0.411064                         | 0.641504                 | blade                        |           |                     |                                                                                       |                                                                                       |                                                                                       |
|      | N1_23                                                                               | 2                                | 2                        | 2                            | 2         |                     |                                                                                       |                                                                                       |                                                                                       |
| 107. | 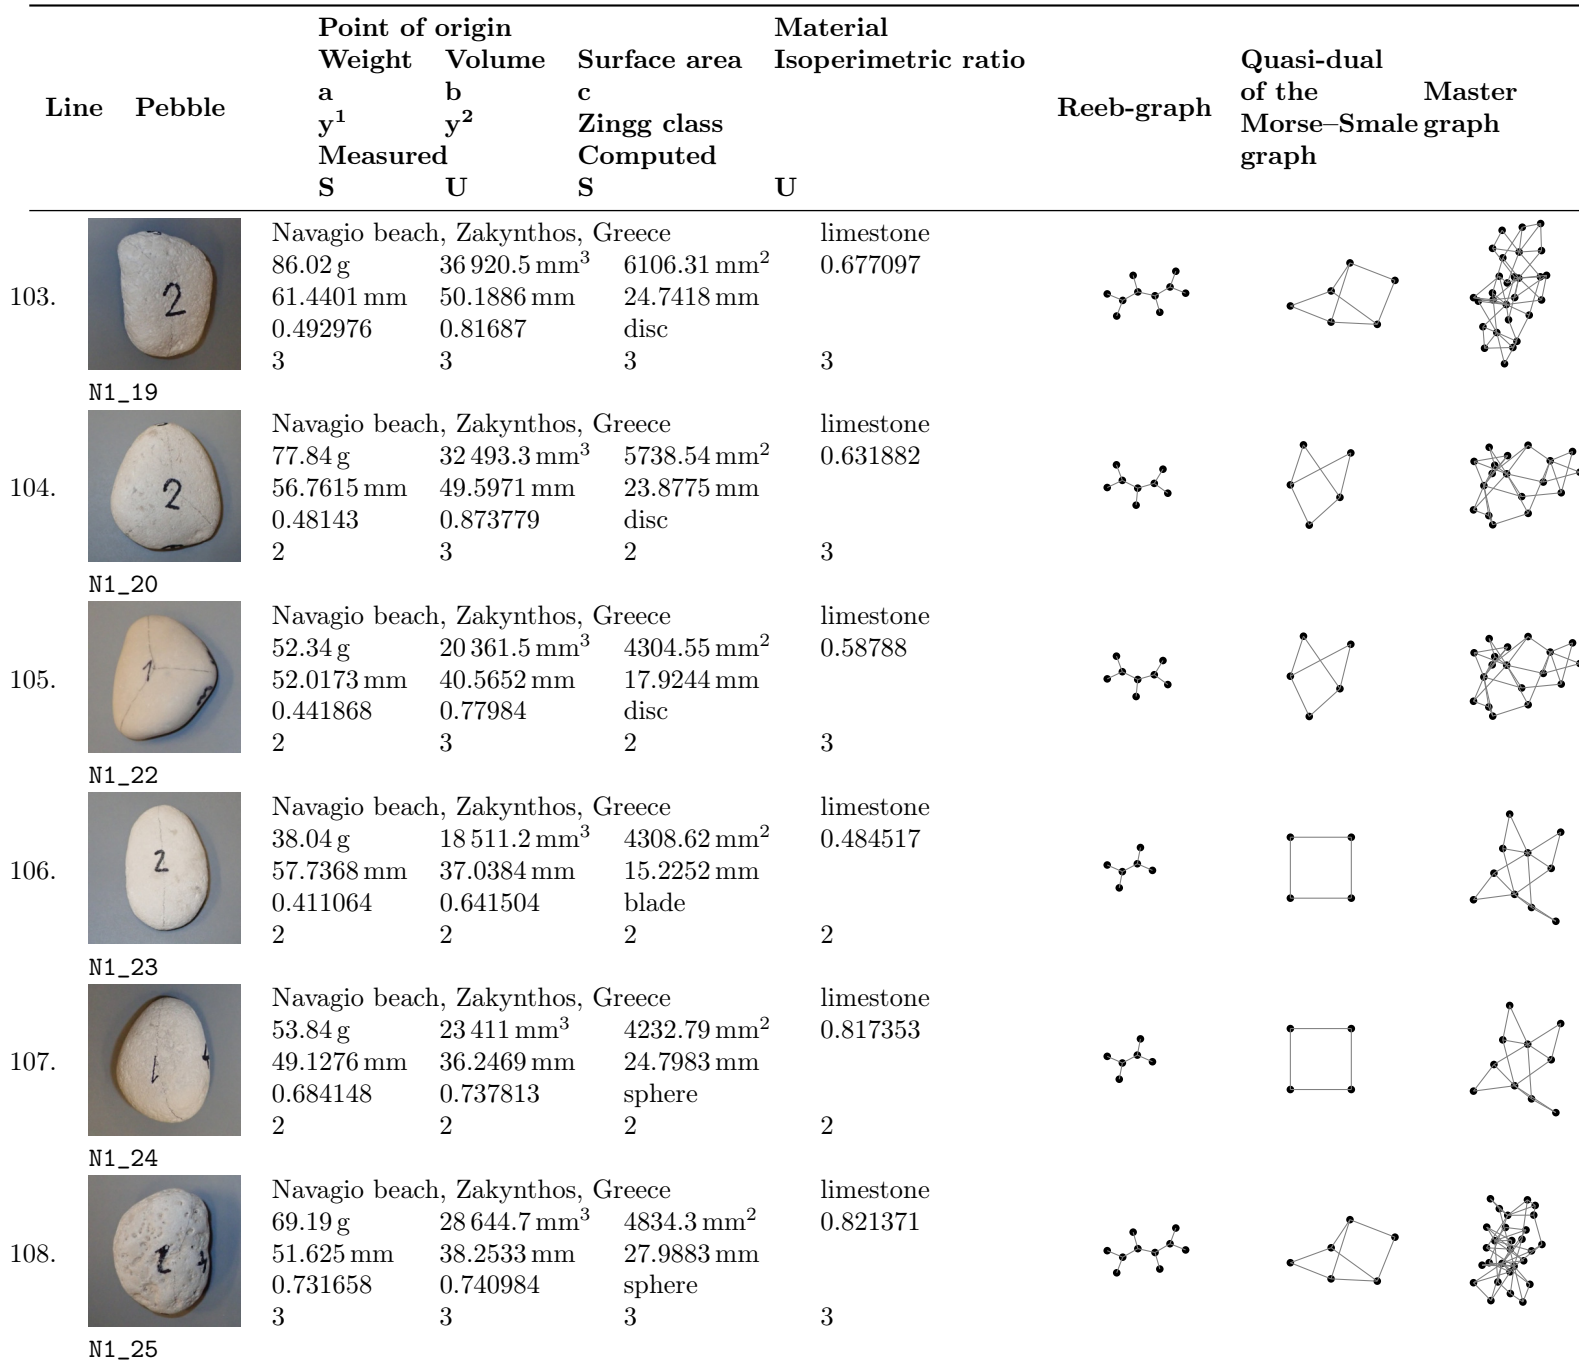 | Navagio beach, Zakynthos, Greece |                          |                              | limestone | 0.817353            | 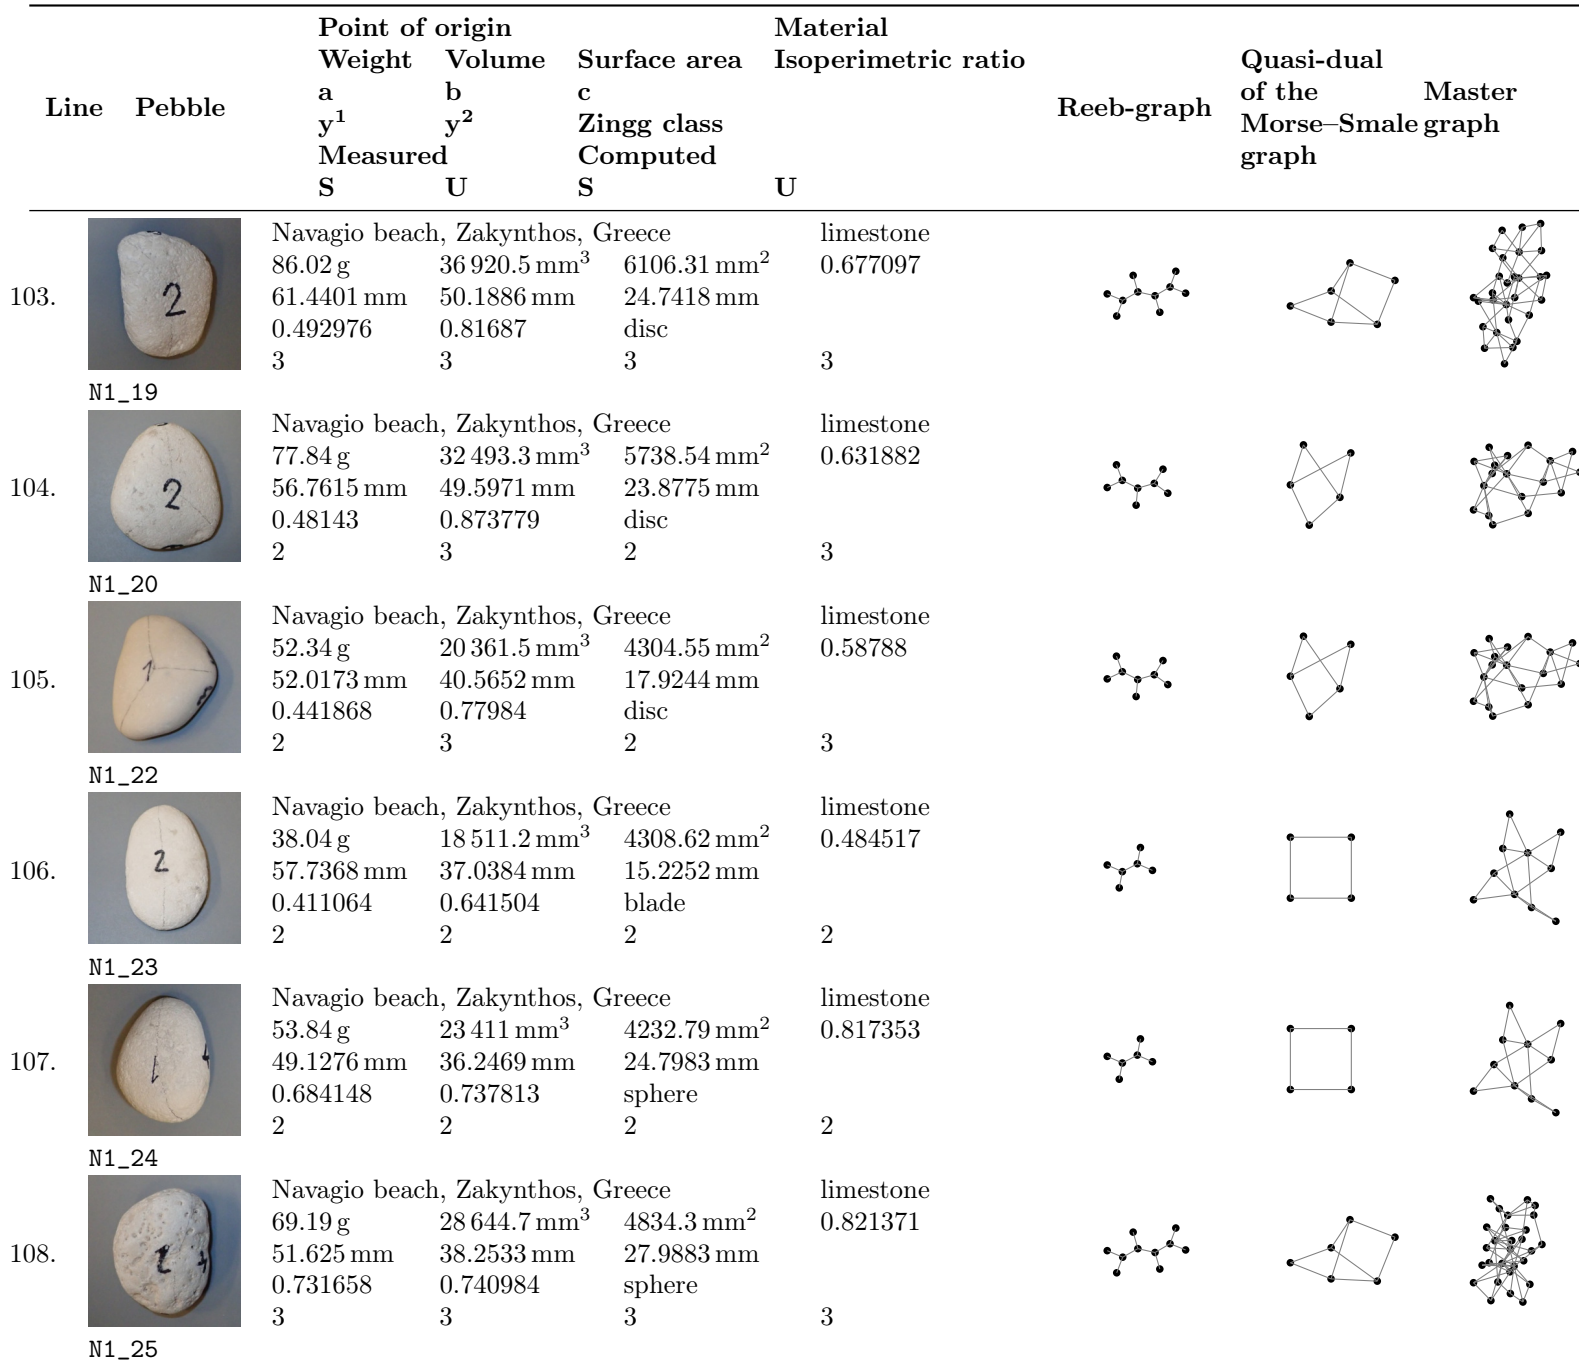 | 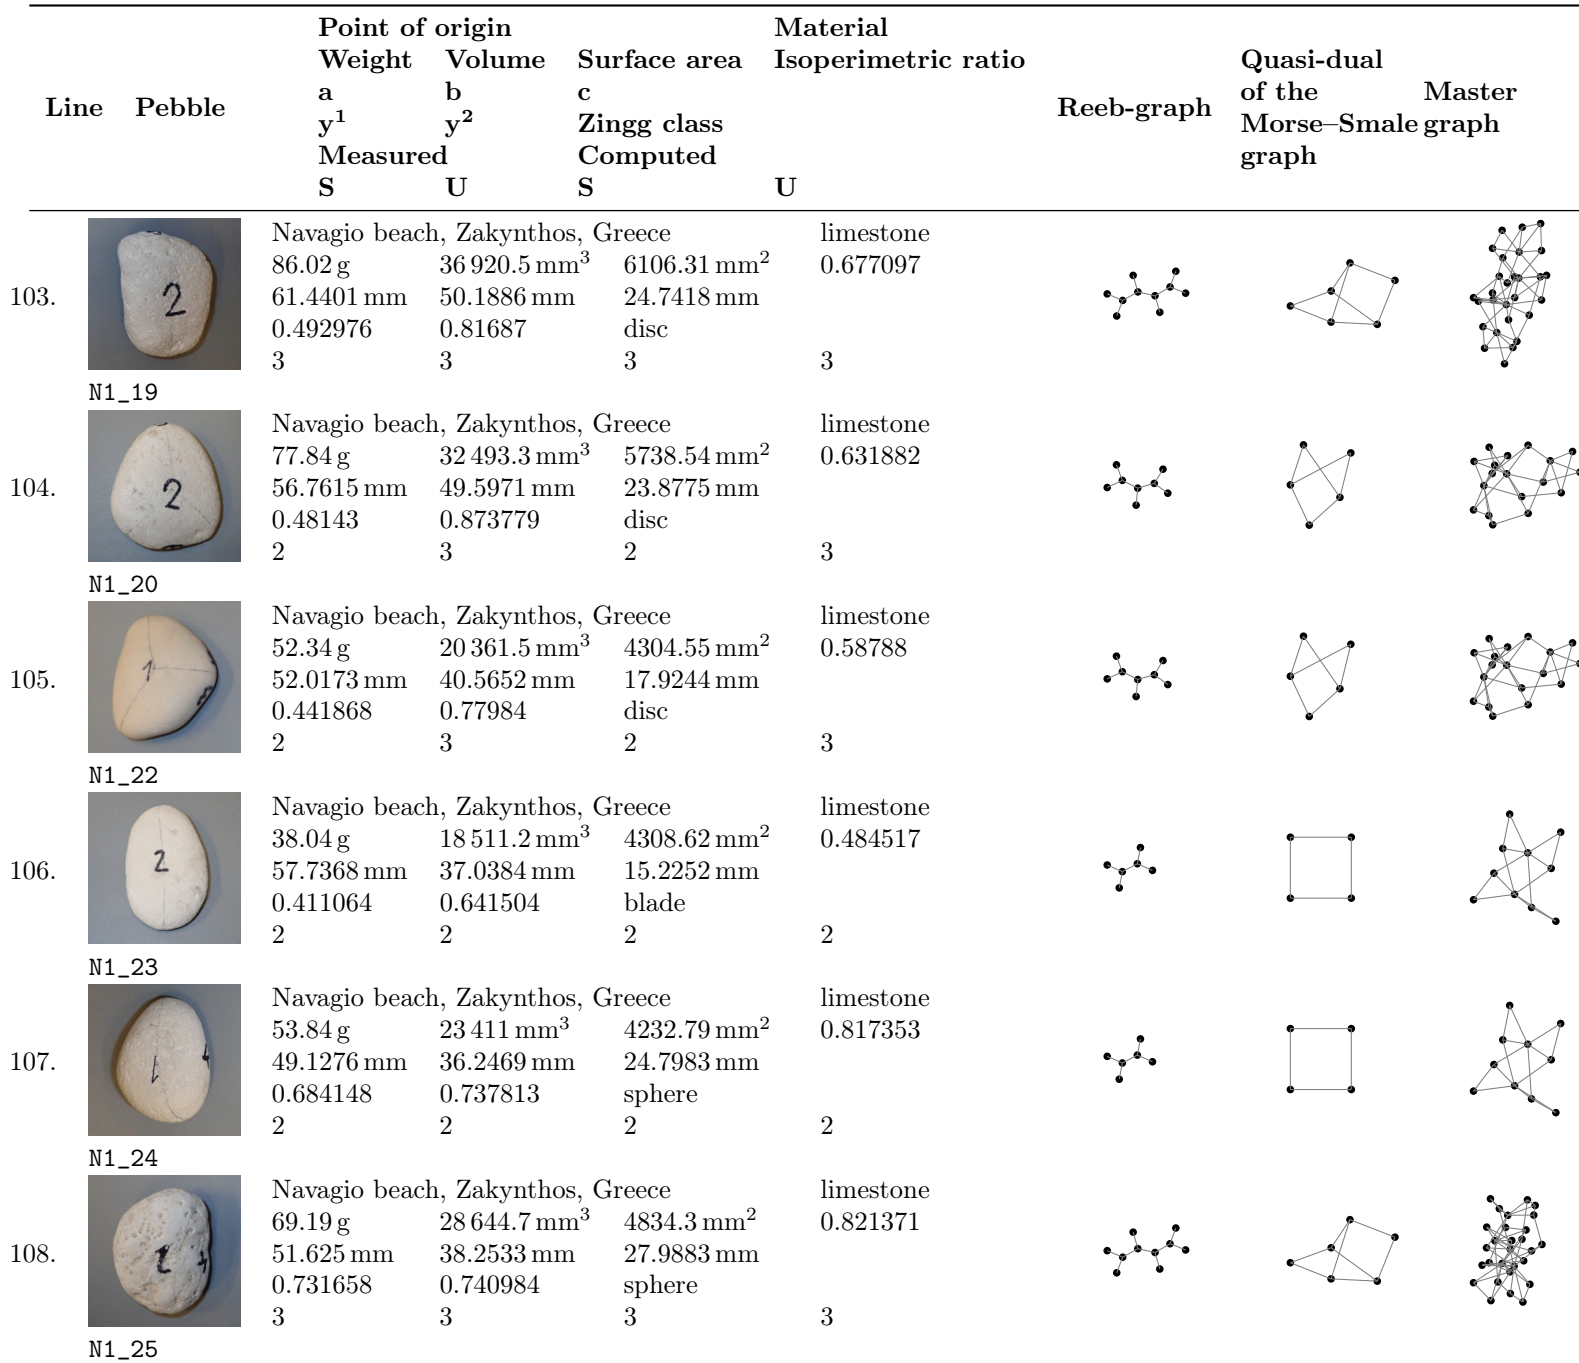 | 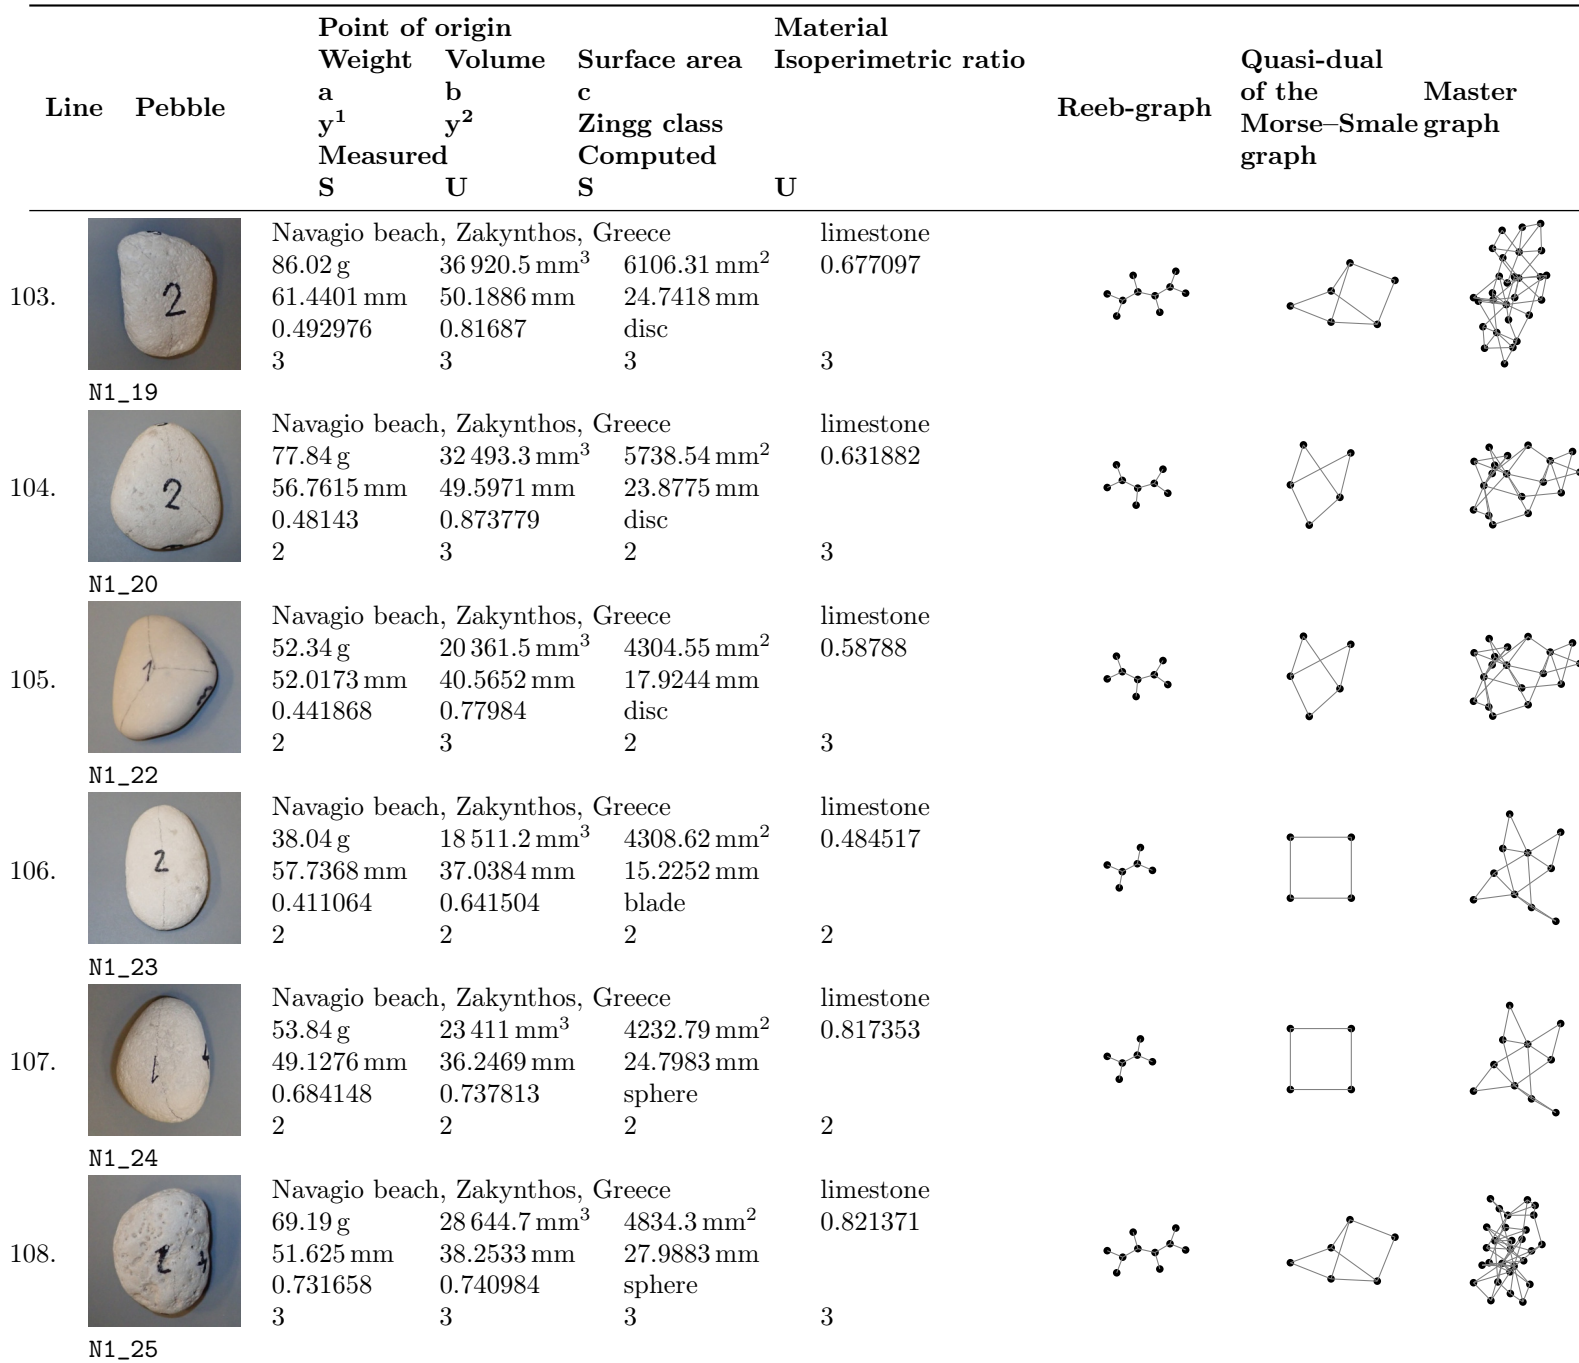 |
|      |                                                                                     | 53.84 g                          | 23 411 mm <sup>3</sup>   | 4232.79 mm <sup>2</sup>      |           |                     |                                                                                       |                                                                                       |                                                                                       |
|      |                                                                                     | 49.1276 mm                       | 36.2469 mm               | 24.7983 mm                   |           |                     |                                                                                       |                                                                                       |                                                                                       |
|      |                                                                                     | 0.684148                         | 0.737813                 | sphere                       |           |                     |                                                                                       |                                                                                       |                                                                                       |
|      | N1_24                                                                               | 2                                | 2                        | 2                            | 2         |                     |                                                                                       |                                                                                       |                                                                                       |
| 108. | 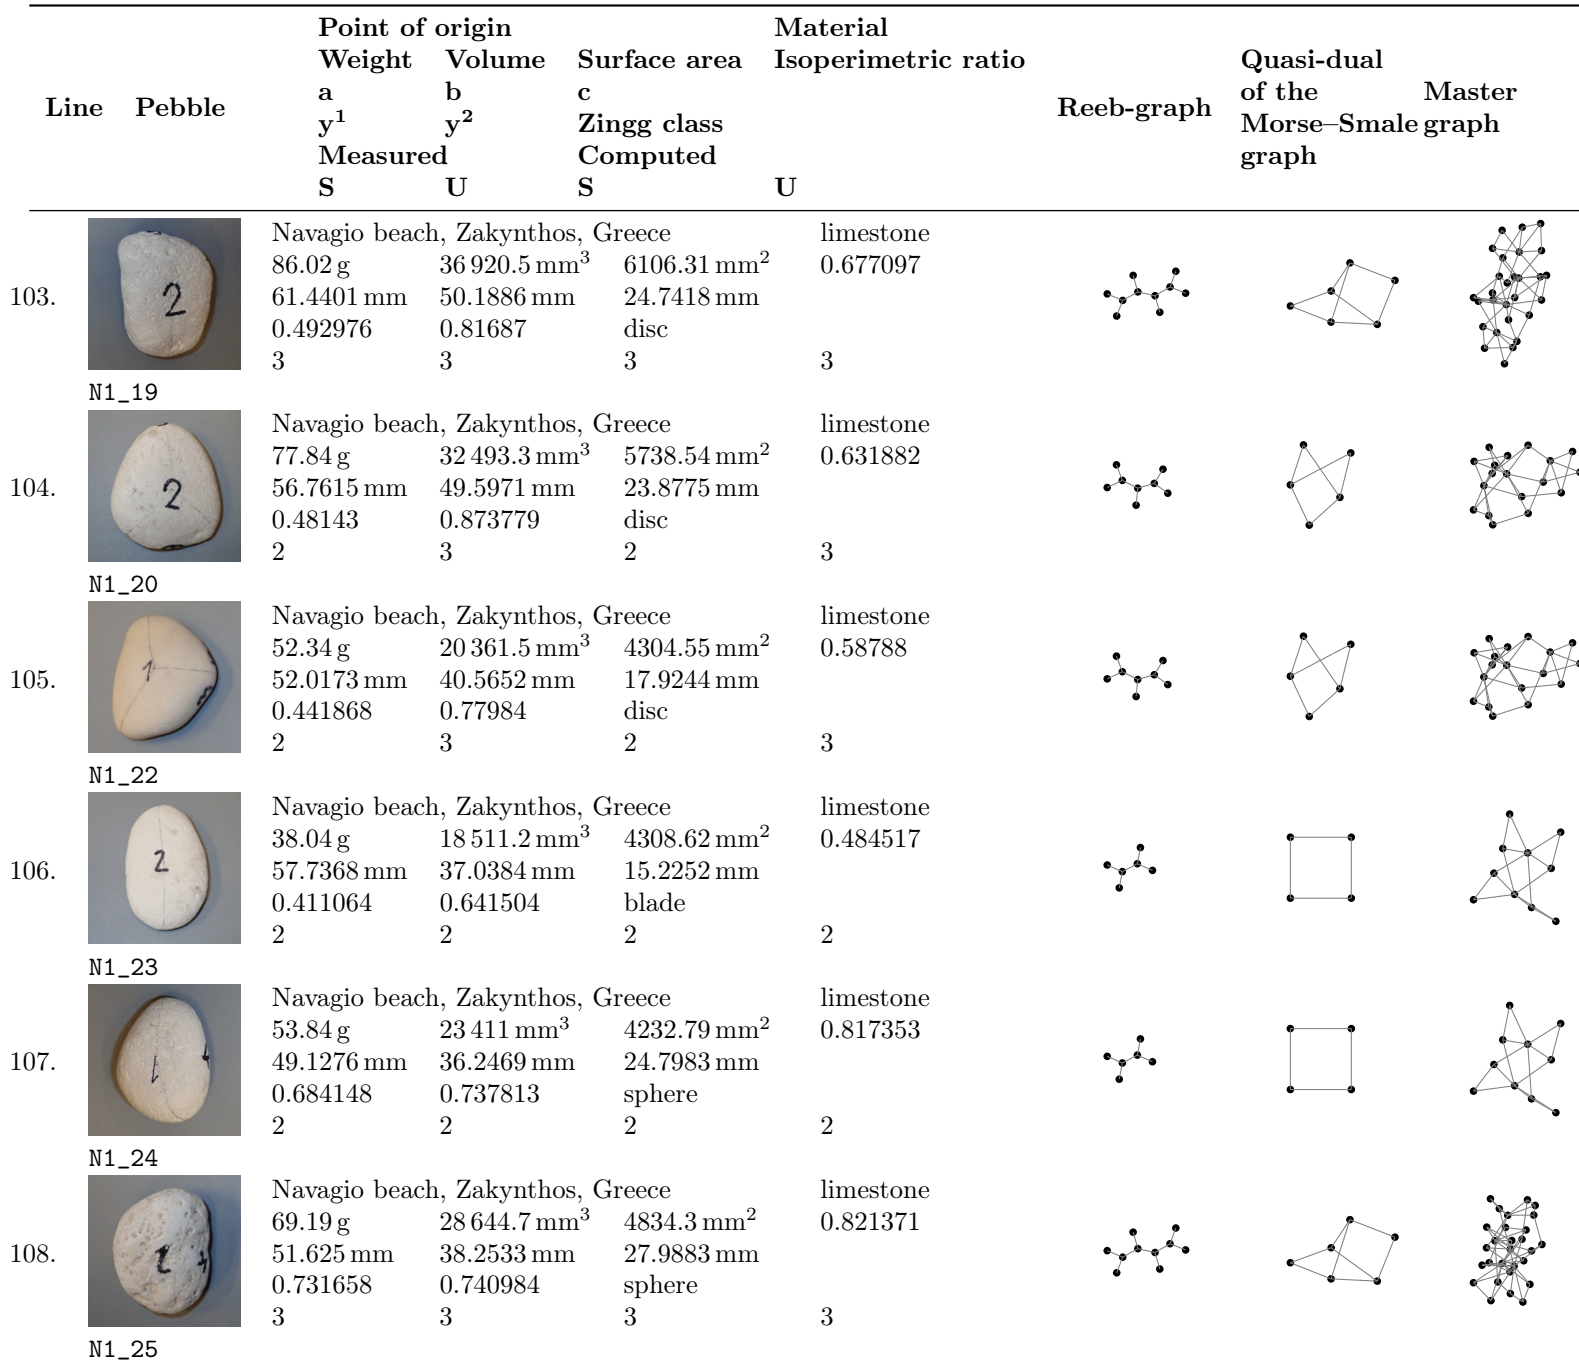 | Navagio beach, Zakynthos, Greece |                          |                              | limestone | 0.821371            | 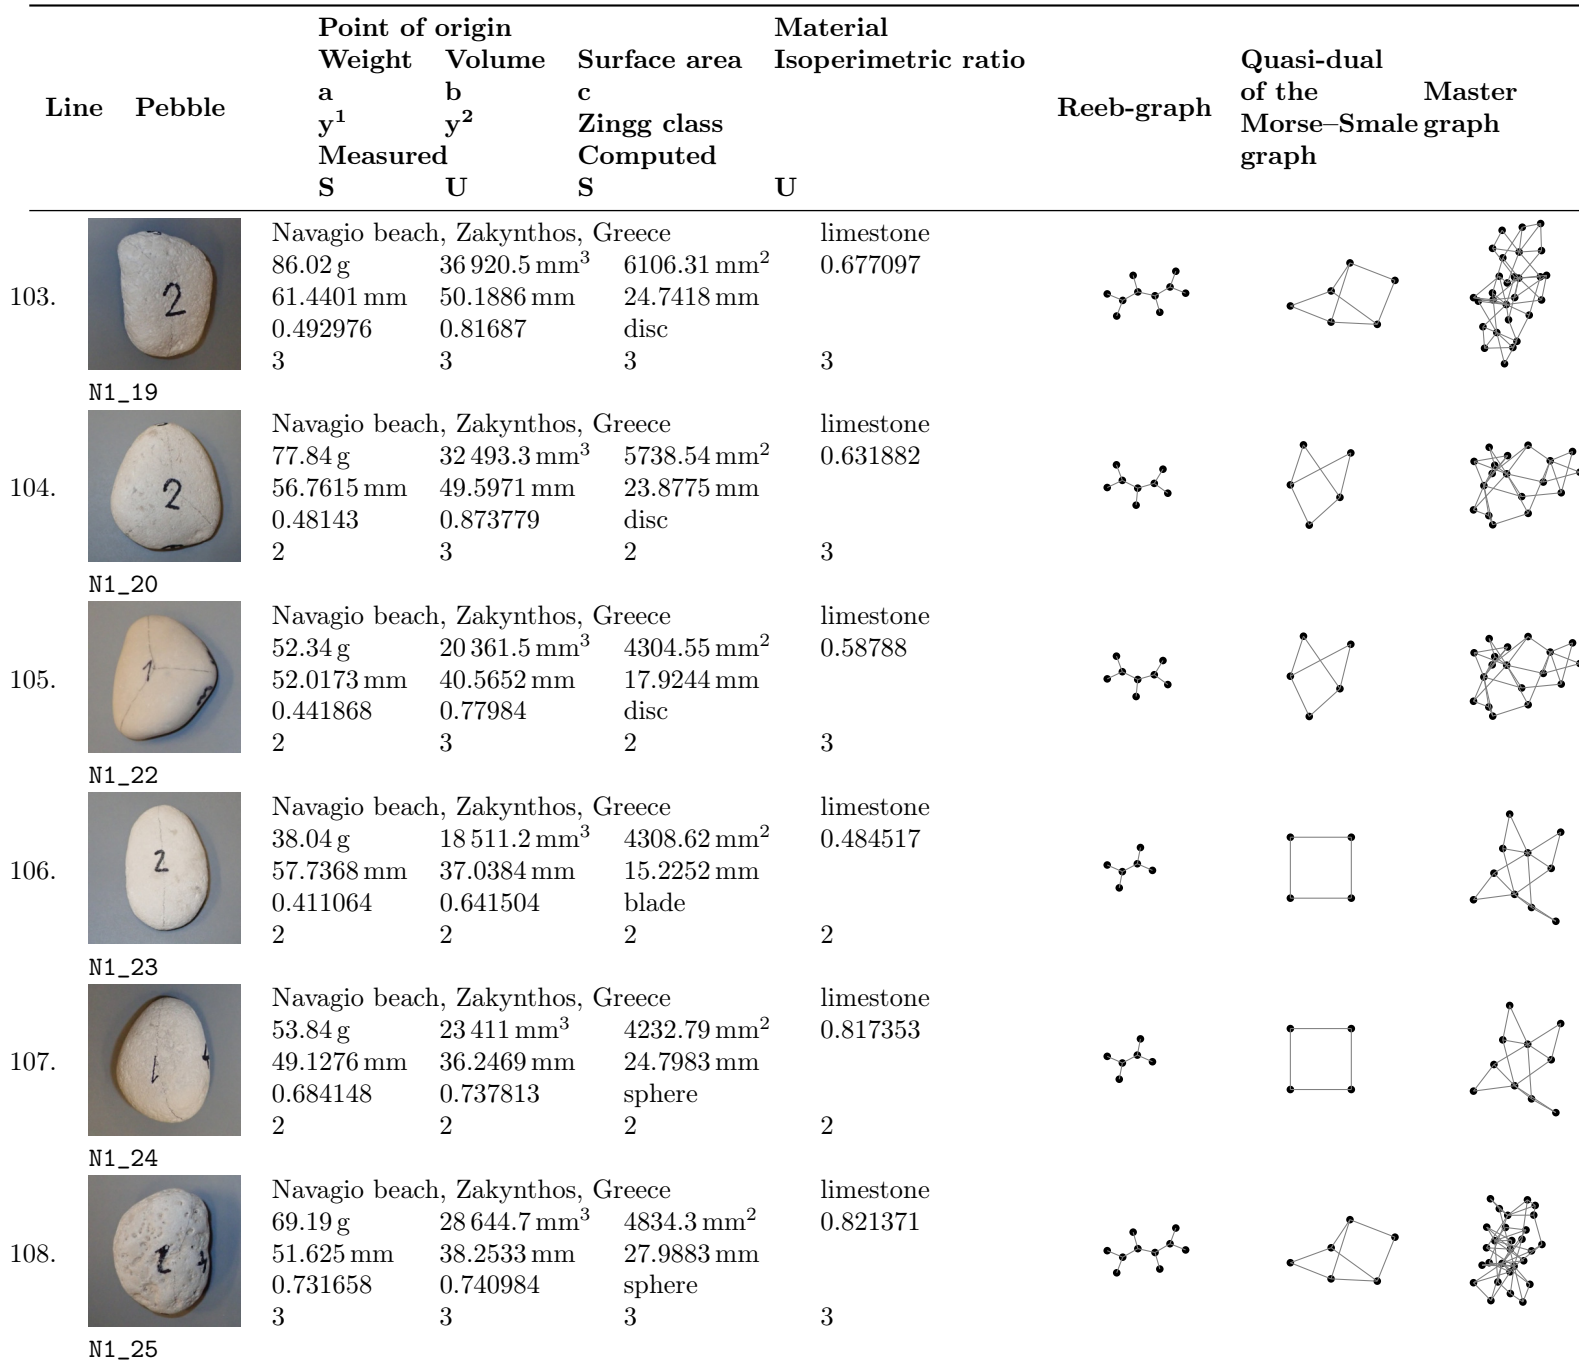 | 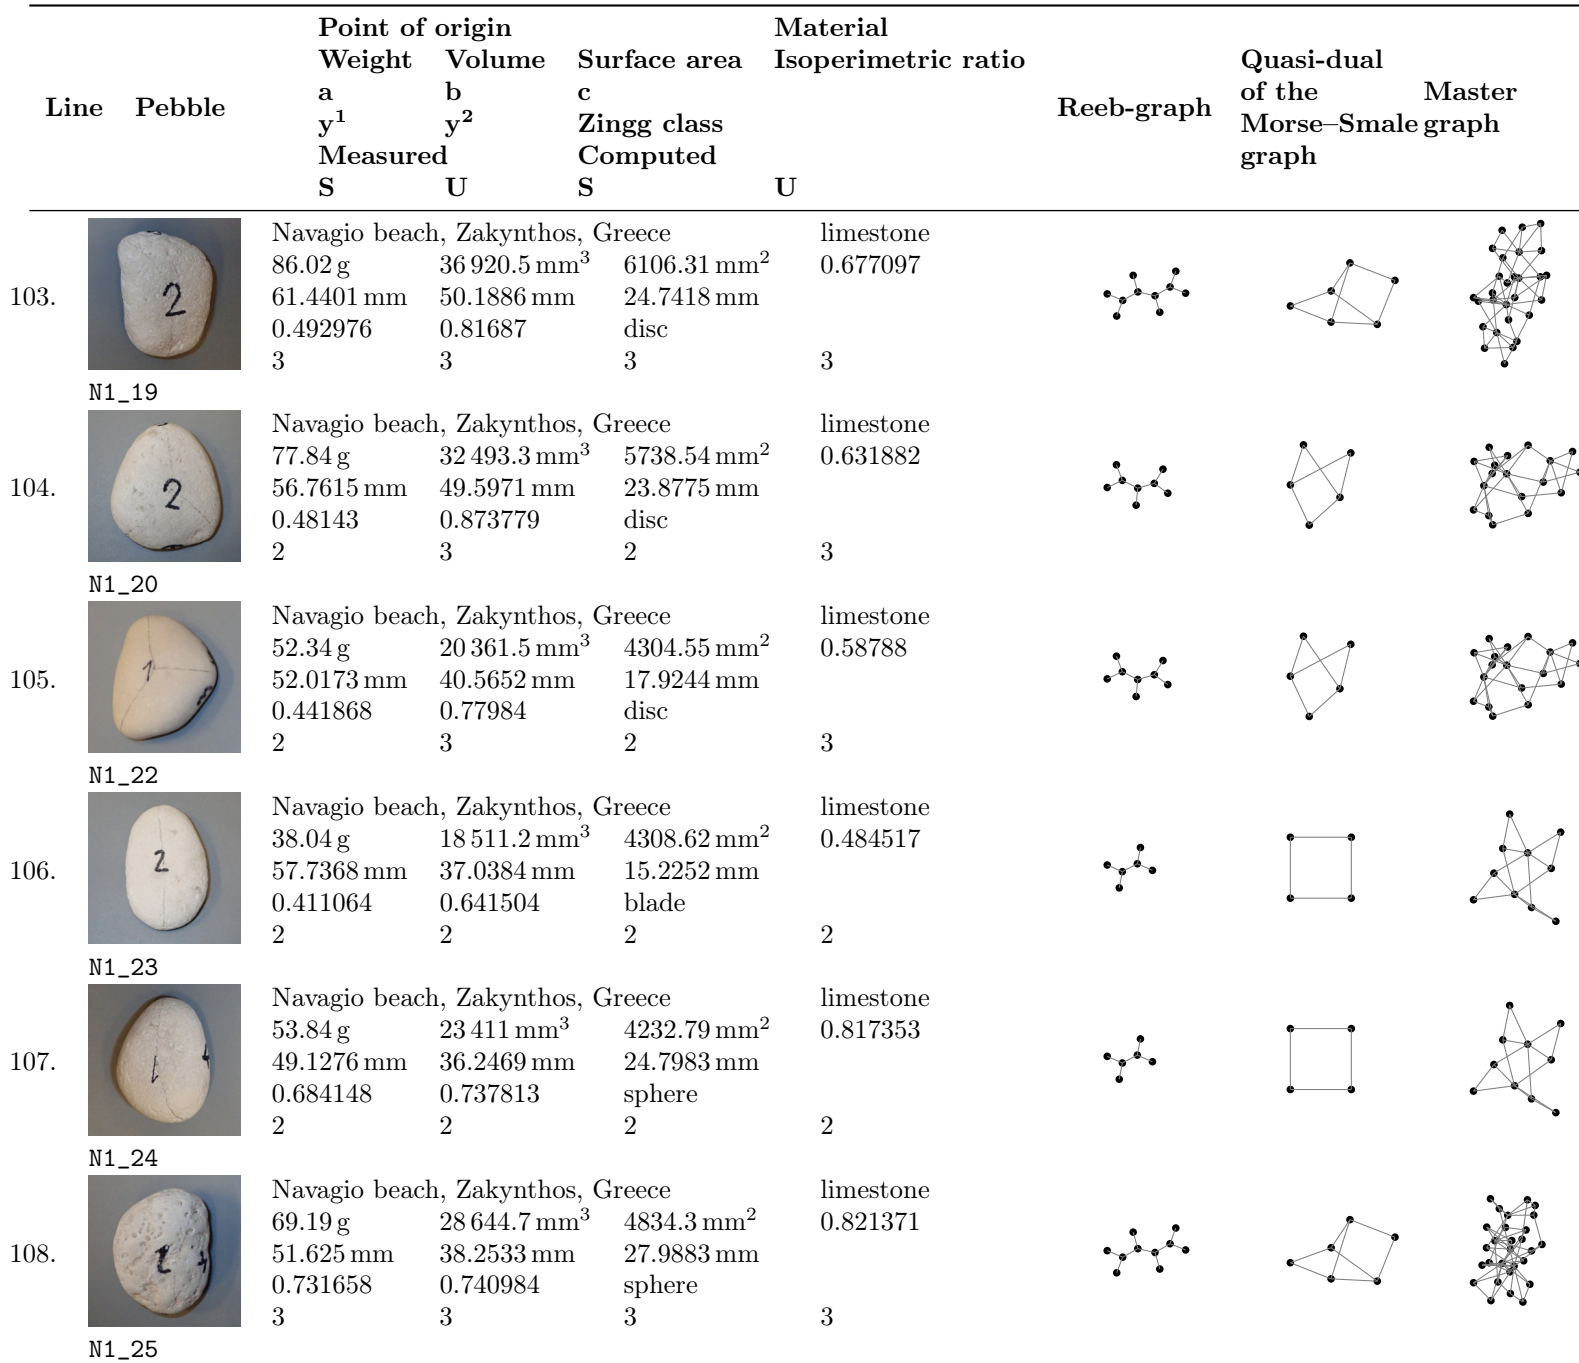 | 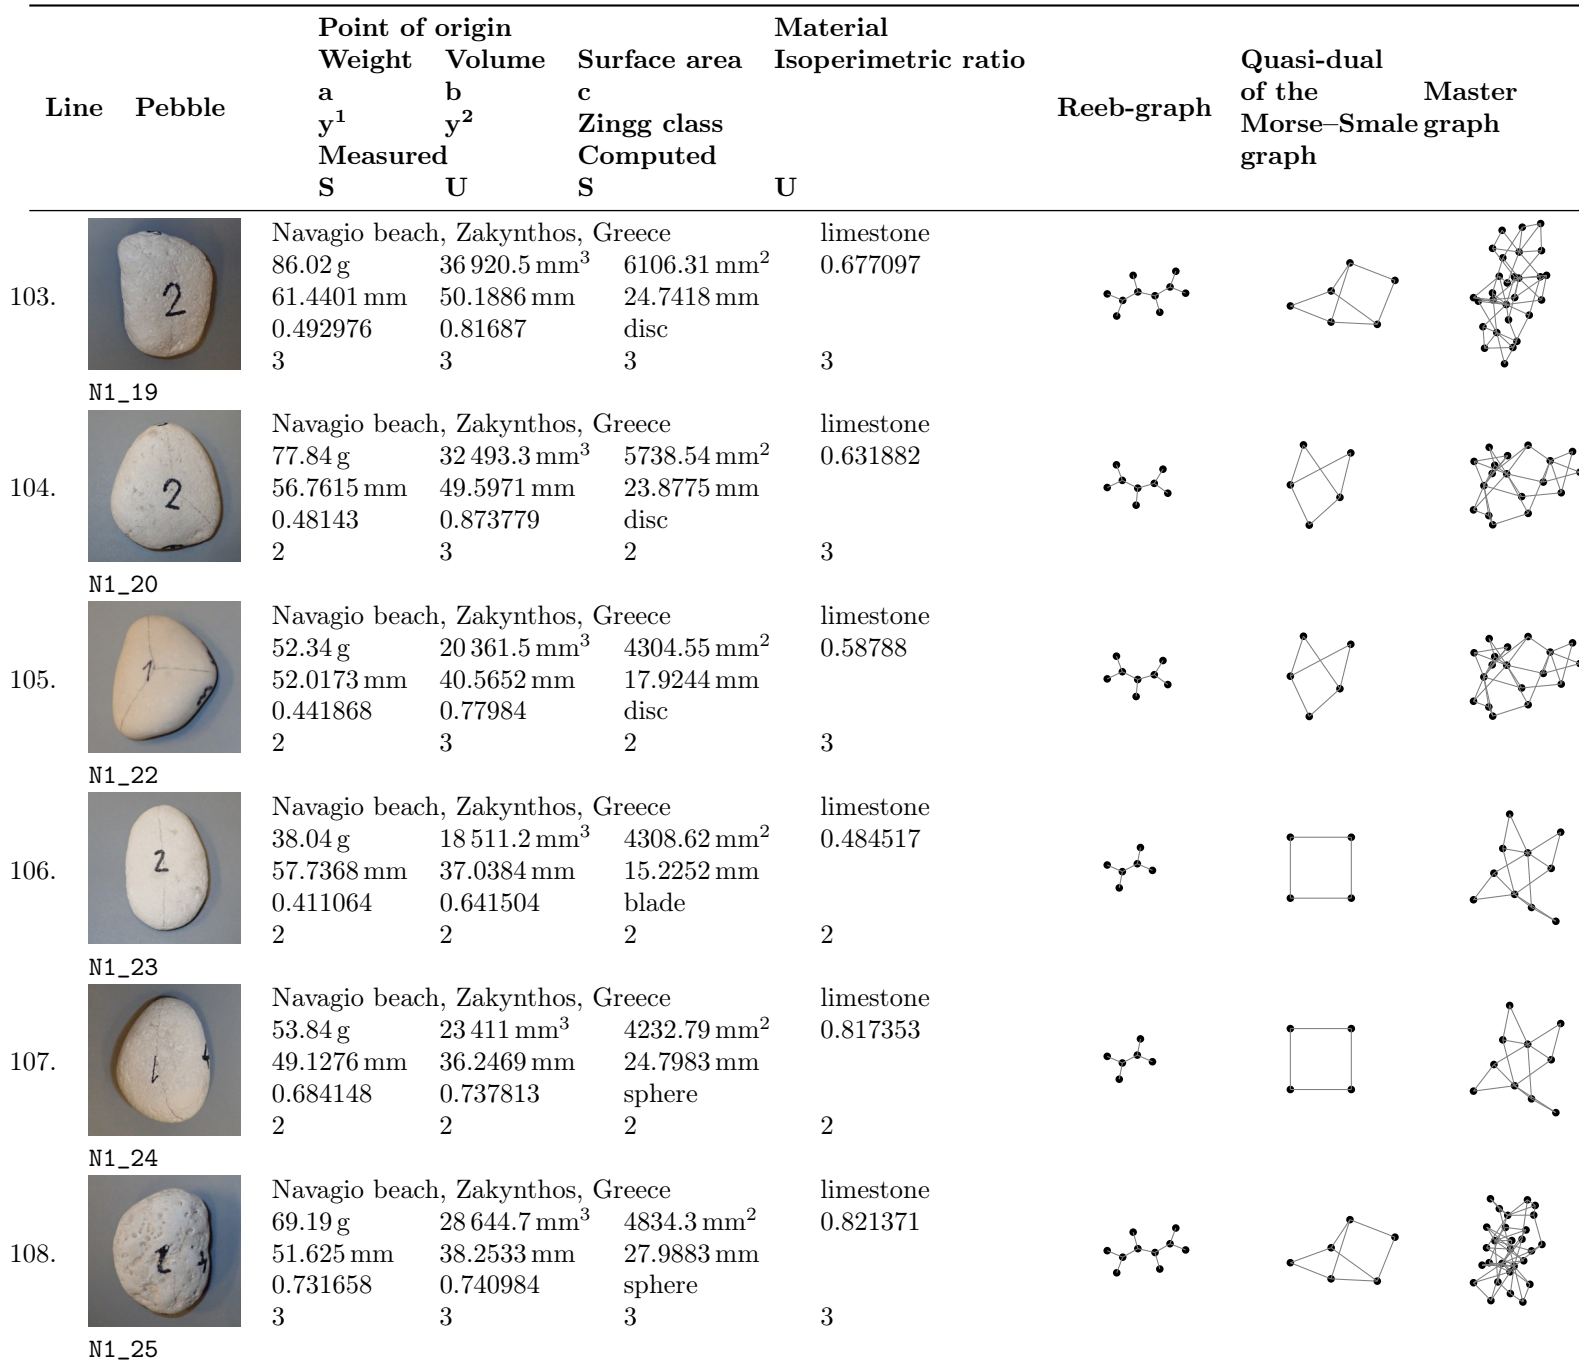 |
|      |                                                                                     | 69.19 g                          | 28 644.7 mm <sup>3</sup> | 4834.3 mm <sup>2</sup>       |           |                     |                                                                                       |                                                                                       |                                                                                       |
|      |                                                                                     | 51.625 mm                        | 38.2533 mm               | 27.9883 mm                   |           |                     |                                                                                       |                                                                                       |                                                                                       |
|      |                                                                                     | 0.731658                         | 0.740984                 | sphere                       |           |                     |                                                                                       |                                                                                       |                                                                                       |
|      | N1_25                                                                               | 3                                | 3                        | 3                            | 3         |                     |                                                                                       |                                                                                       |                                                                                       |

| Line | Pebble                                                                              | Point of origin                  |                          |                         | Material  | Isoperimetric ratio | Reeb-graph | Quasi-dual<br>of the<br>Morse–Smale<br>graph | Master<br>graph |
|------|-------------------------------------------------------------------------------------|----------------------------------|--------------------------|-------------------------|-----------|---------------------|------------|----------------------------------------------|-----------------|
|      |                                                                                     | Weight                           | Volume                   | Surface area            |           |                     |            |                                              |                 |
|      |                                                                                     | a                                | b                        | c                       |           |                     |            |                                              |                 |
|      |                                                                                     | y <sup>1</sup>                   | y <sup>2</sup>           | Zingg class             |           |                     |            |                                              |                 |
|      |                                                                                     | Measured                         |                          | Computed                |           |                     |            |                                              |                 |
|      |                                                                                     | S                                | U                        | S                       | U         |                     |            |                                              |                 |
| 109. | 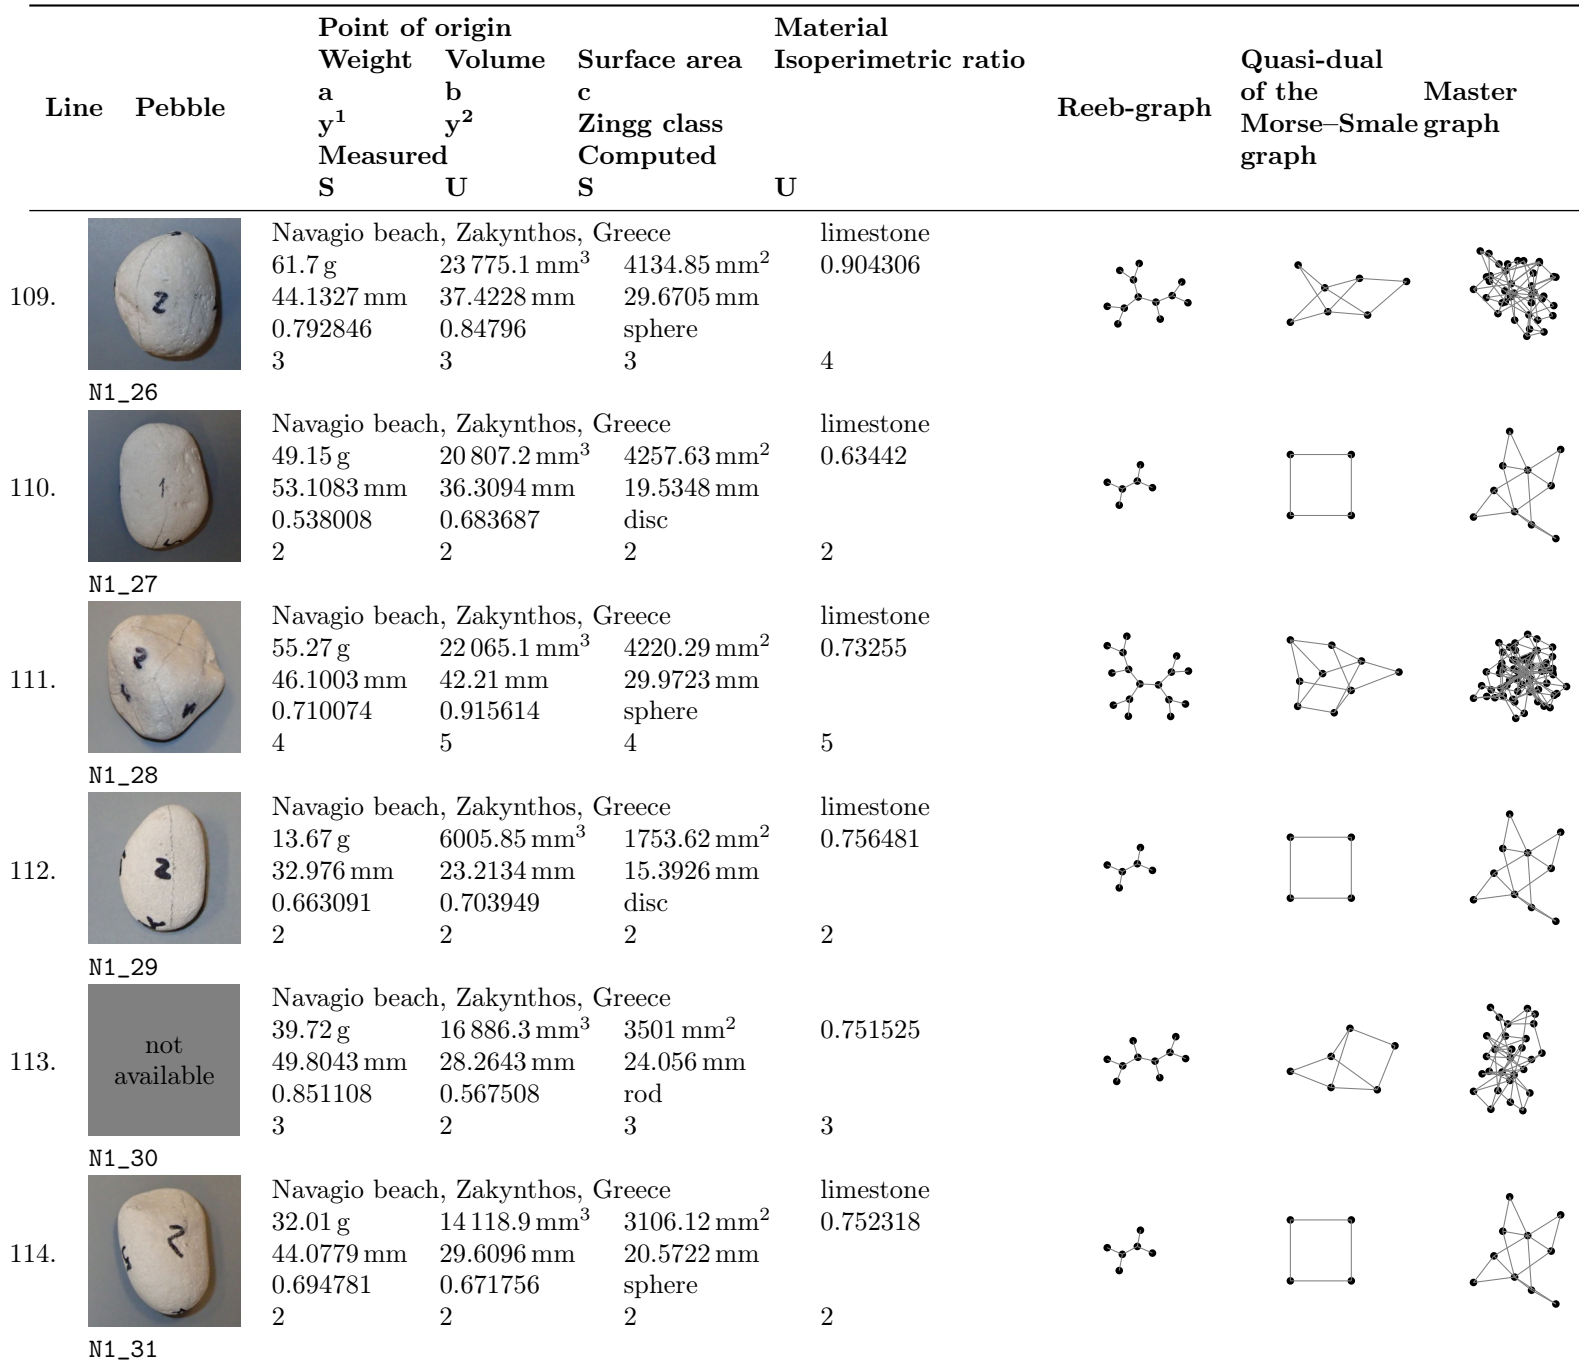   | Navagio beach, Zakynthos, Greece |                          |                         | limestone |                     |            |                                              |                 |
|      |                                                                                     | 61.7 g                           | 23 775.1 mm <sup>3</sup> | 4134.85 mm <sup>2</sup> | 0.904306  |                     |            |                                              |                 |
|      |                                                                                     | 44.1327 mm                       | 37.4228 mm               | 29.6705 mm              |           |                     |            |                                              |                 |
|      |                                                                                     | 0.792846                         | 0.84796                  | sphere                  |           |                     |            |                                              |                 |
|      |                                                                                     | 3                                | 3                        | 3                       | 4         |                     |            |                                              |                 |
|      |                                                                                     | N1_26                            |                          |                         |           |                     |            |                                              |                 |
| 110. | 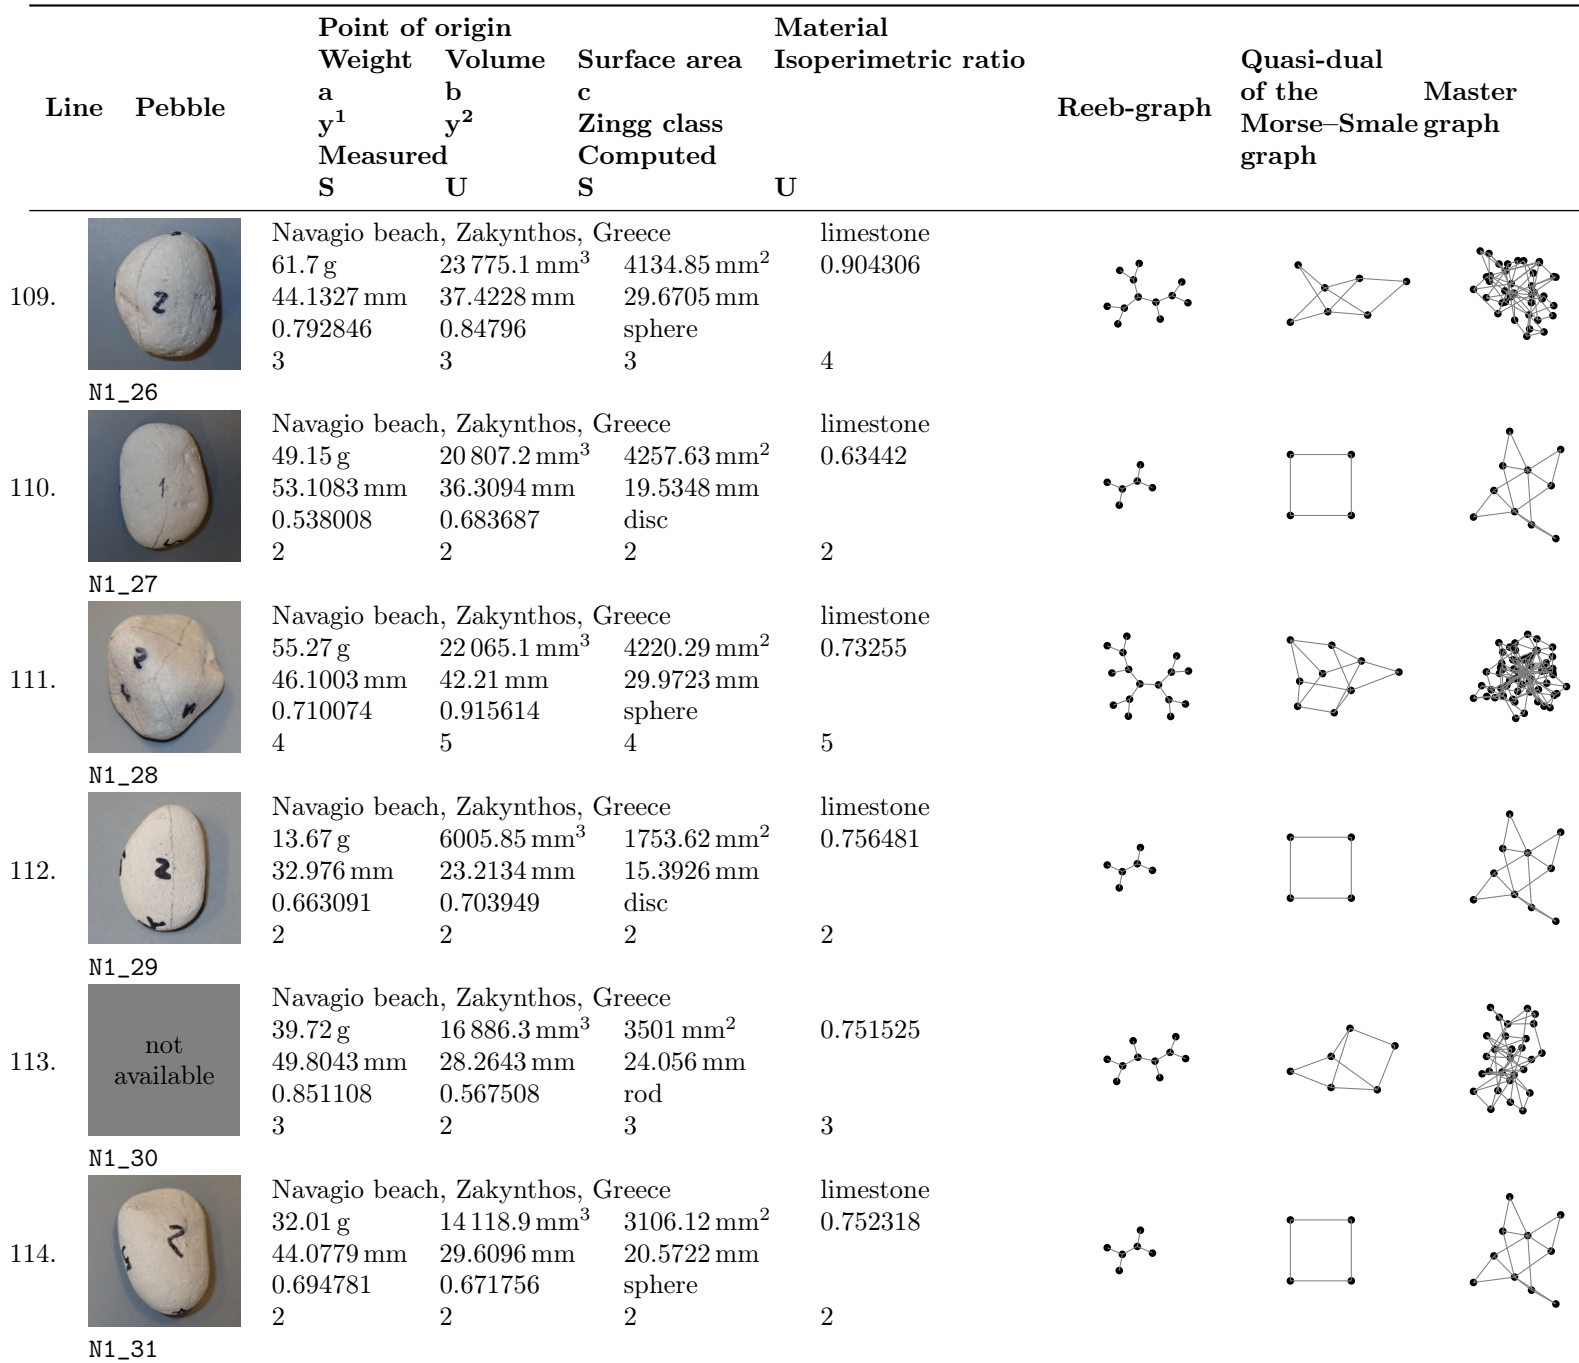   | Navagio beach, Zakynthos, Greece |                          |                         | limestone |                     |            |                                              |                 |
|      |                                                                                     | 49.15 g                          | 20 807.2 mm <sup>3</sup> | 4257.63 mm <sup>2</sup> | 0.63442   |                     |            |                                              |                 |
|      |                                                                                     | 53.1083 mm                       | 36.3094 mm               | 19.5348 mm              |           |                     |            |                                              |                 |
|      |                                                                                     | 0.538008                         | 0.683687                 | disc                    |           |                     |            |                                              |                 |
|      |                                                                                     | 2                                | 2                        | 2                       | 2         |                     |            |                                              |                 |
|      |                                                                                     | N1_27                            |                          |                         |           |                     |            |                                              |                 |
| 111. | 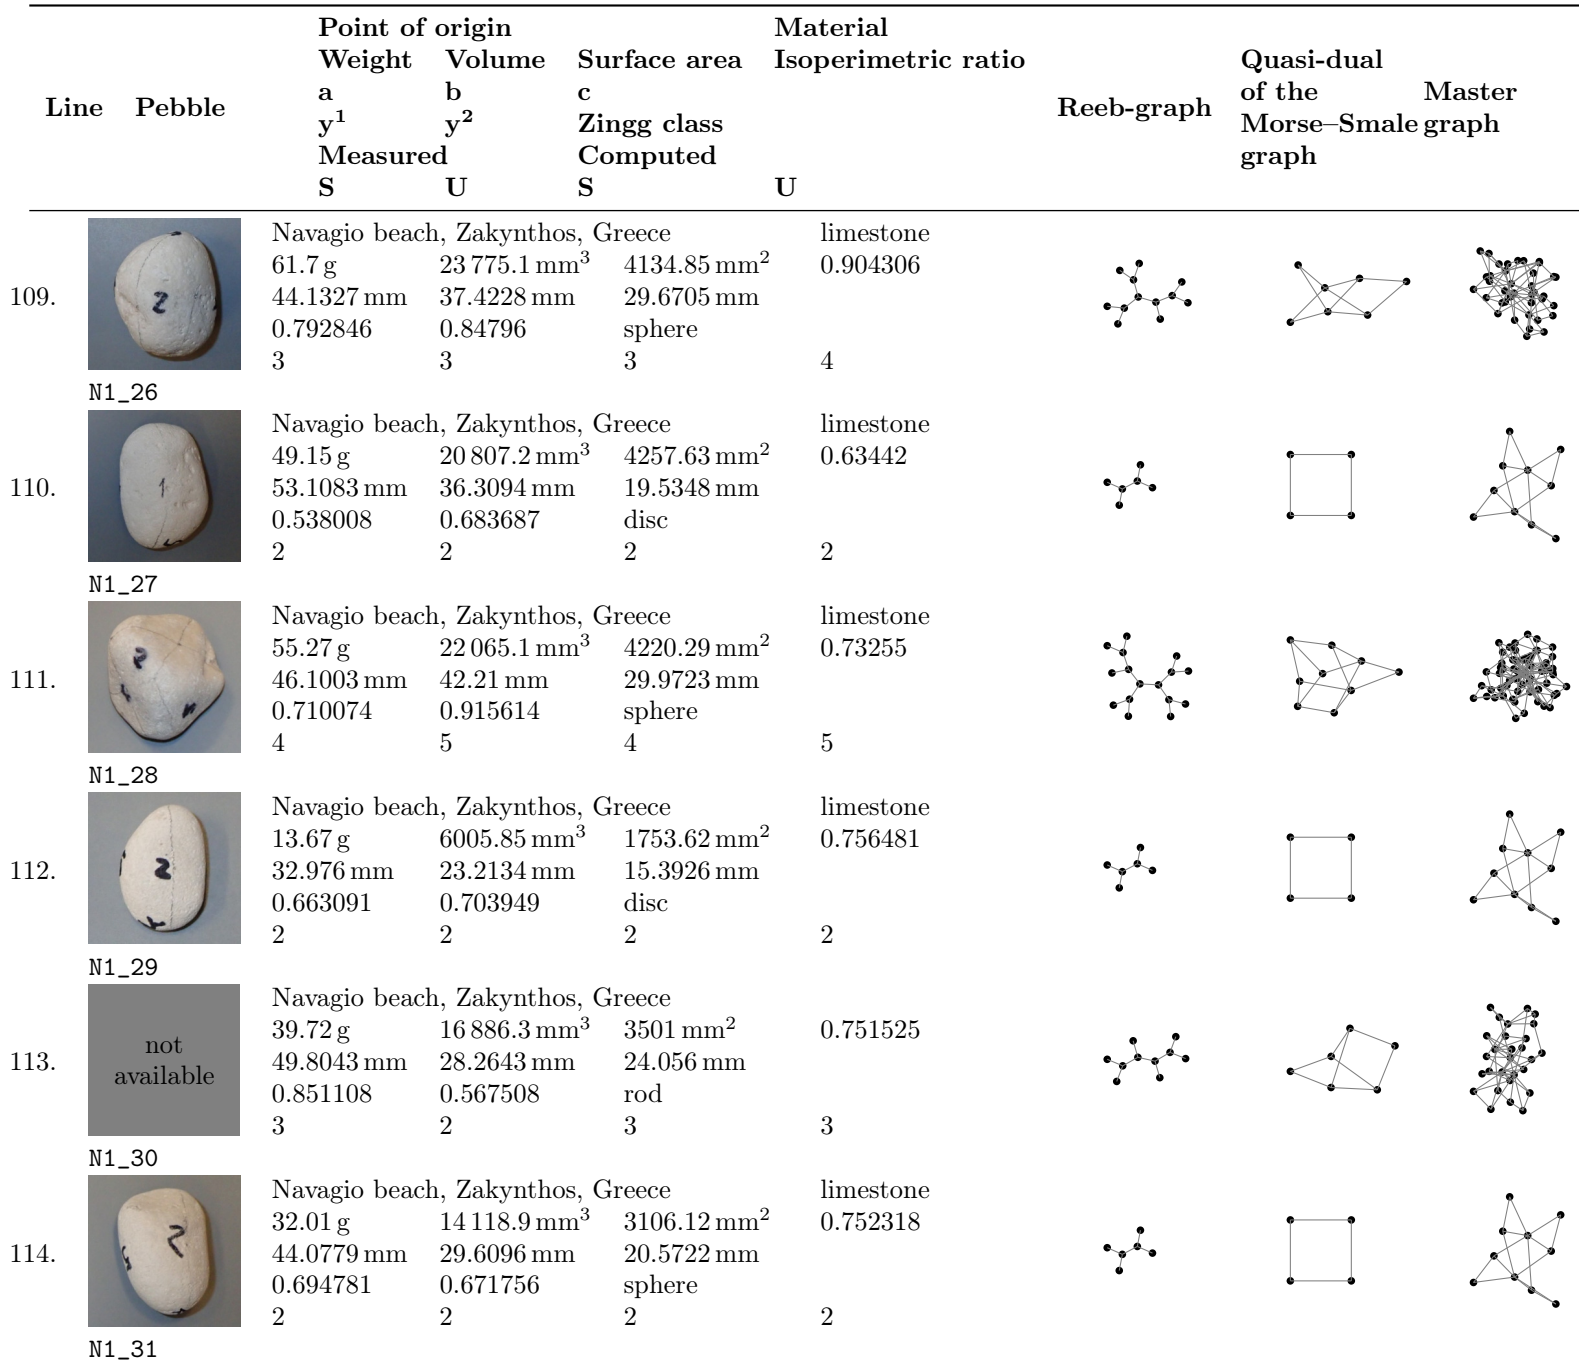   | Navagio beach, Zakynthos, Greece |                          |                         | limestone |                     |            |                                              |                 |
|      |                                                                                     | 55.27 g                          | 22 065.1 mm <sup>3</sup> | 4220.29 mm <sup>2</sup> | 0.73255   |                     |            |                                              |                 |
|      |                                                                                     | 46.1003 mm                       | 42.21 mm                 | 29.9723 mm              |           |                     |            |                                              |                 |
|      |                                                                                     | 0.710074                         | 0.915614                 | sphere                  |           |                     |            |                                              |                 |
|      |                                                                                     | 4                                | 5                        | 4                       | 5         |                     |            |                                              |                 |
|      |                                                                                     | N1_28                            |                          |                         |           |                     |            |                                              |                 |
| 112. | 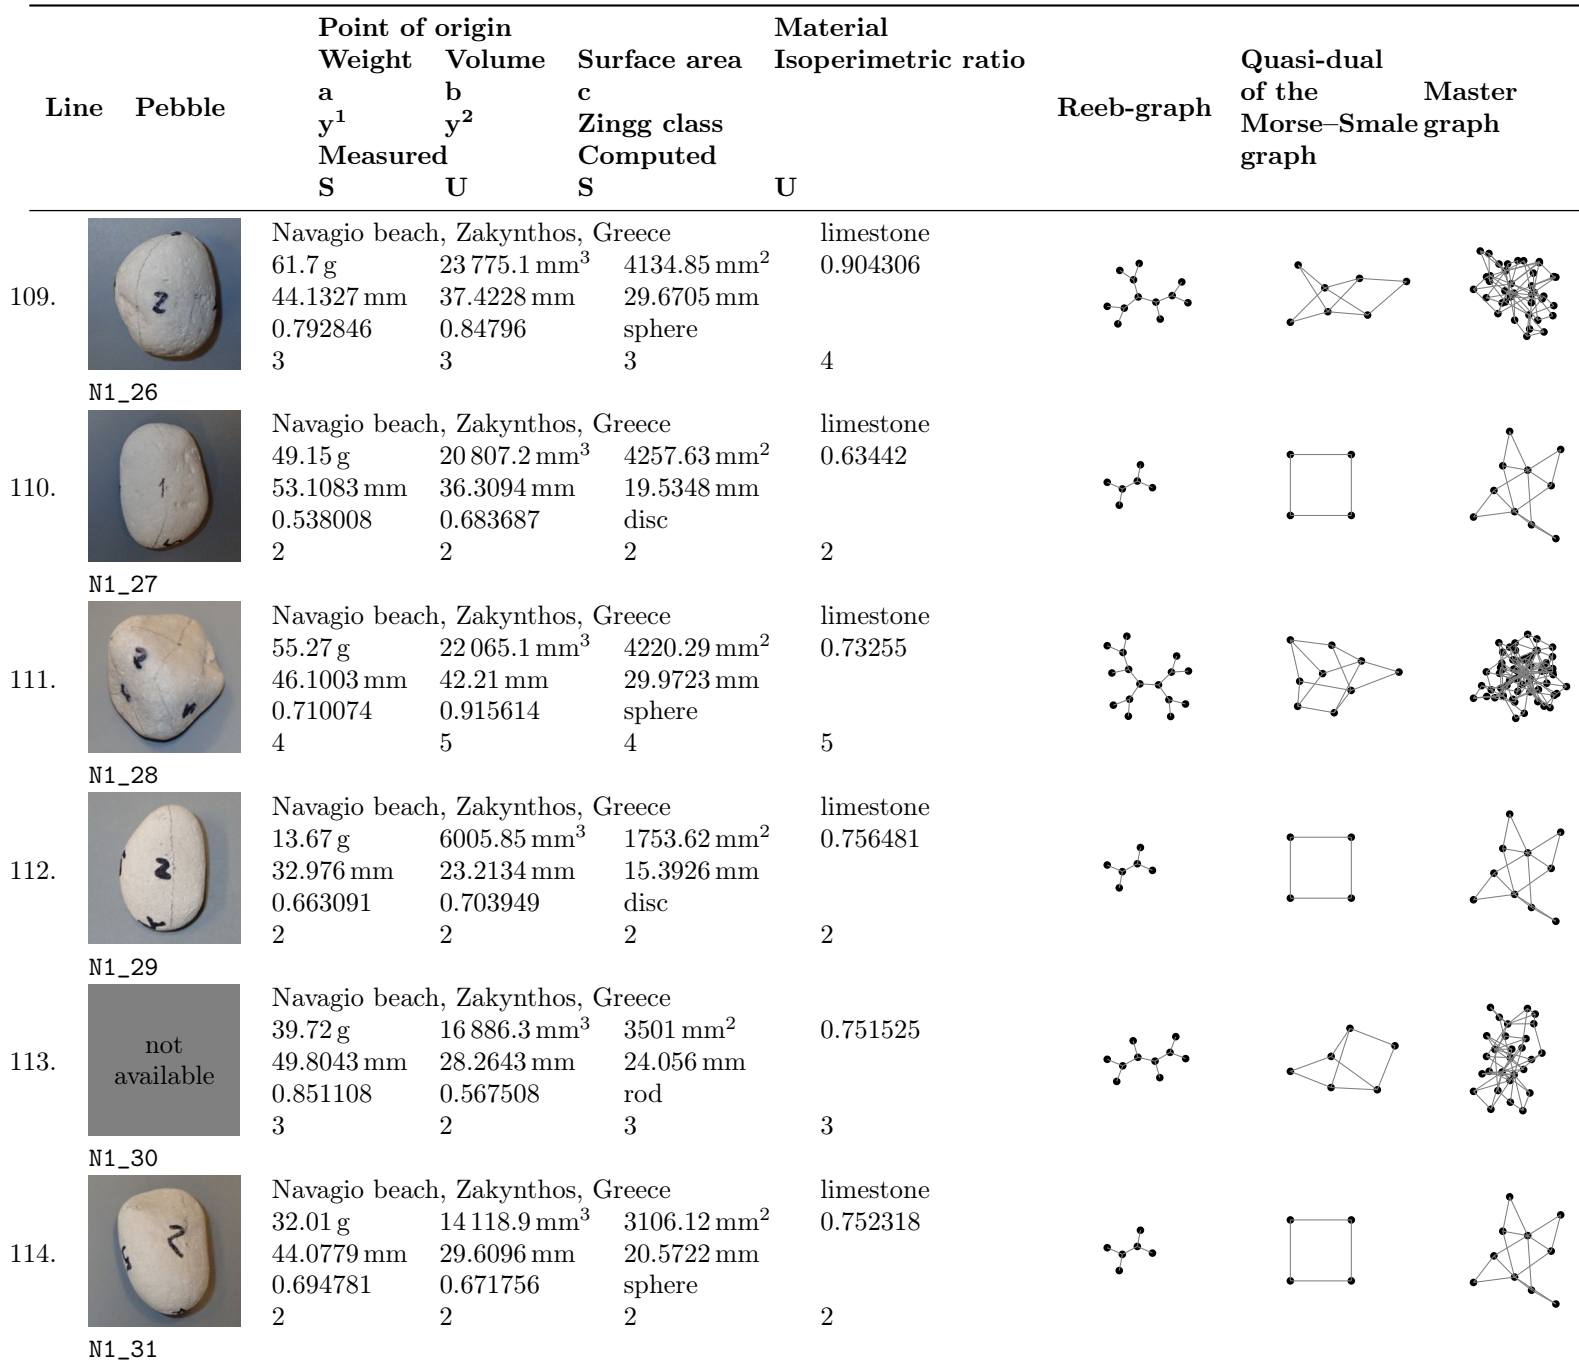  | Navagio beach, Zakynthos, Greece |                          |                         | limestone |                     |            |                                              |                 |
|      |                                                                                     | 13.67 g                          | 6005.85 mm <sup>3</sup>  | 1753.62 mm <sup>2</sup> | 0.756481  |                     |            |                                              |                 |
|      |                                                                                     | 32.976 mm                        | 23.2134 mm               | 15.3926 mm              |           |                     |            |                                              |                 |
|      |                                                                                     | 0.663091                         | 0.703949                 | disc                    |           |                     |            |                                              |                 |
|      |                                                                                     | 2                                | 2                        | 2                       | 2         |                     |            |                                              |                 |
|      |                                                                                     | N1_29                            |                          |                         |           |                     |            |                                              |                 |
| 113. | 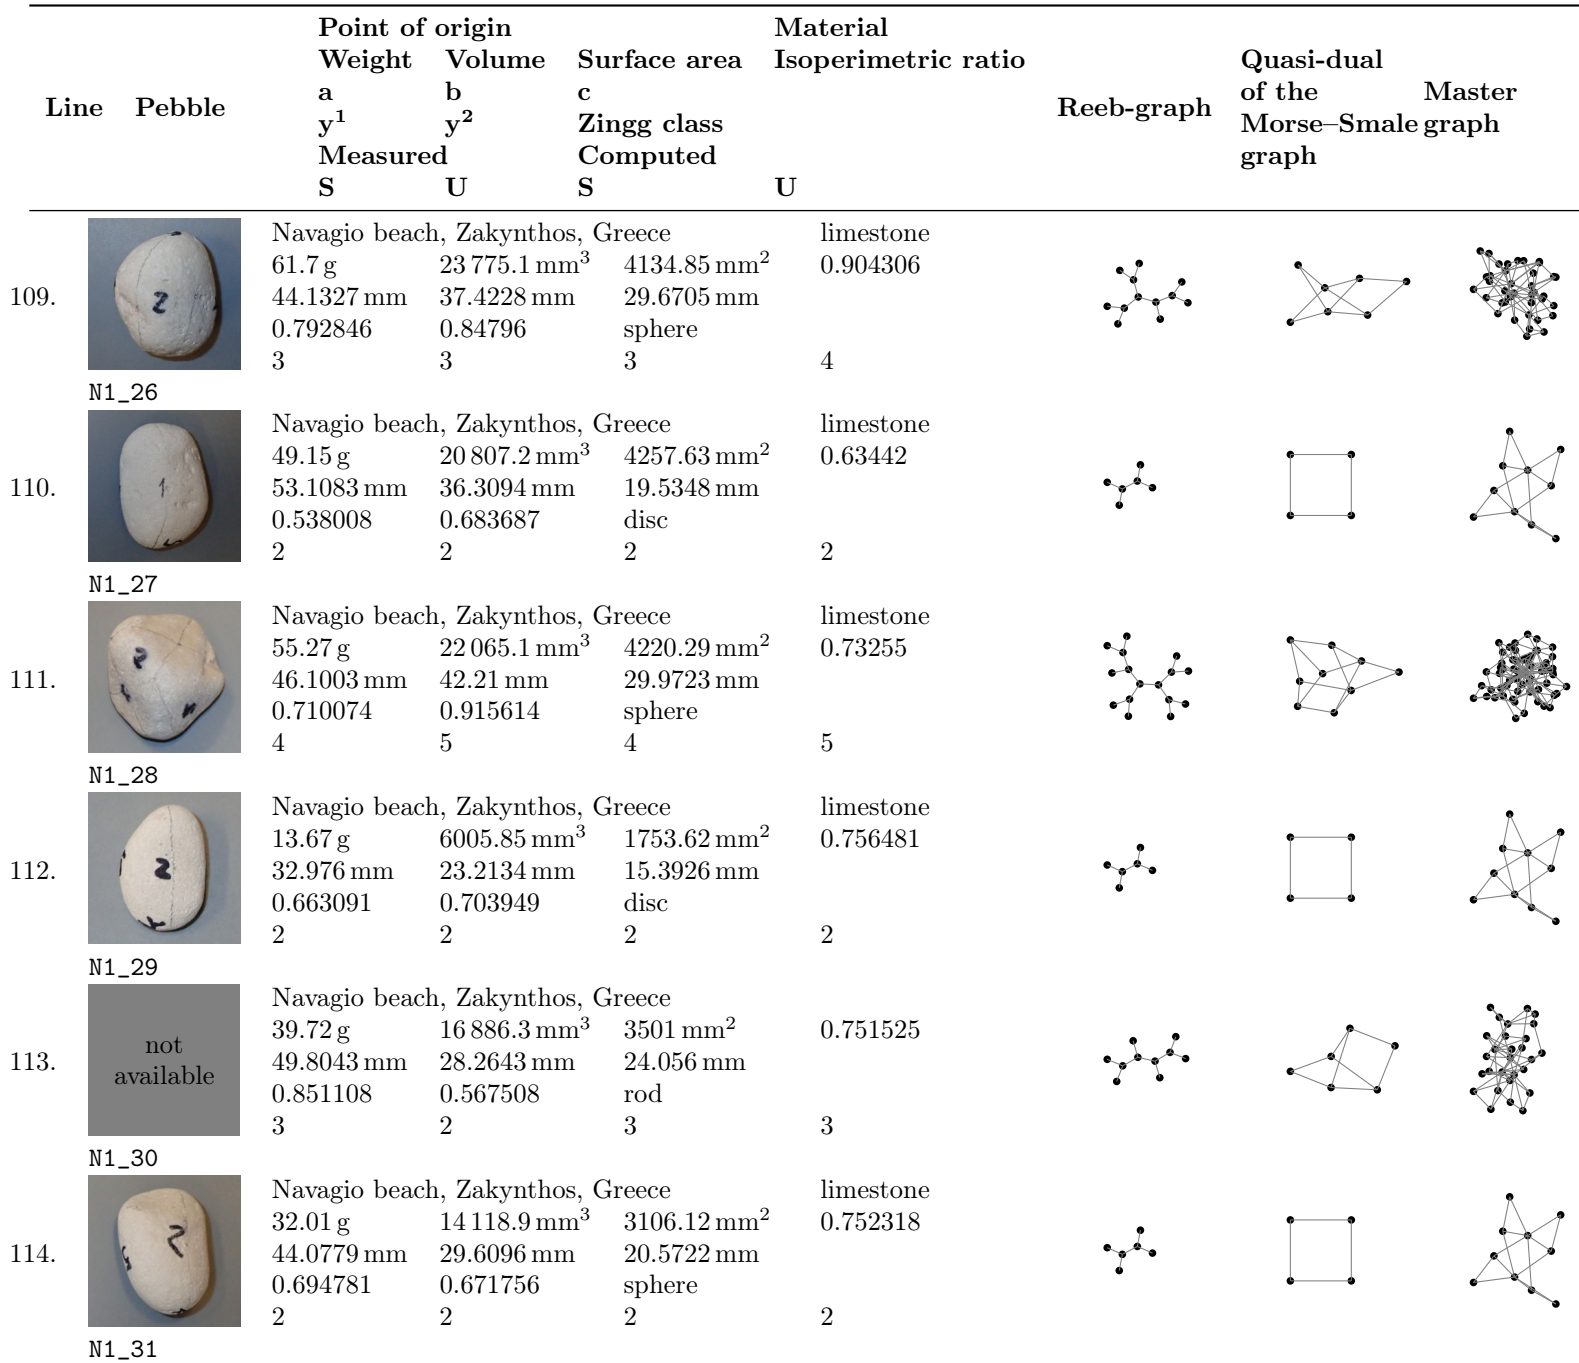 | Navagio beach, Zakynthos, Greece |                          |                         |           |                     |            |                                              |                 |
|      |                                                                                     | 39.72 g                          | 16 886.3 mm <sup>3</sup> | 3501 mm <sup>2</sup>    | 0.751525  |                     |            |                                              |                 |
|      |                                                                                     | 49.8043 mm                       | 28.2643 mm               | 24.056 mm               |           |                     |            |                                              |                 |
|      |                                                                                     | 0.851108                         | 0.567508                 | rod                     |           |                     |            |                                              |                 |
|      |                                                                                     | 3                                | 2                        | 3                       | 3         |                     |            |                                              |                 |
|      |                                                                                     | N1_30                            |                          |                         |           |                     |            |                                              |                 |
| 114. | 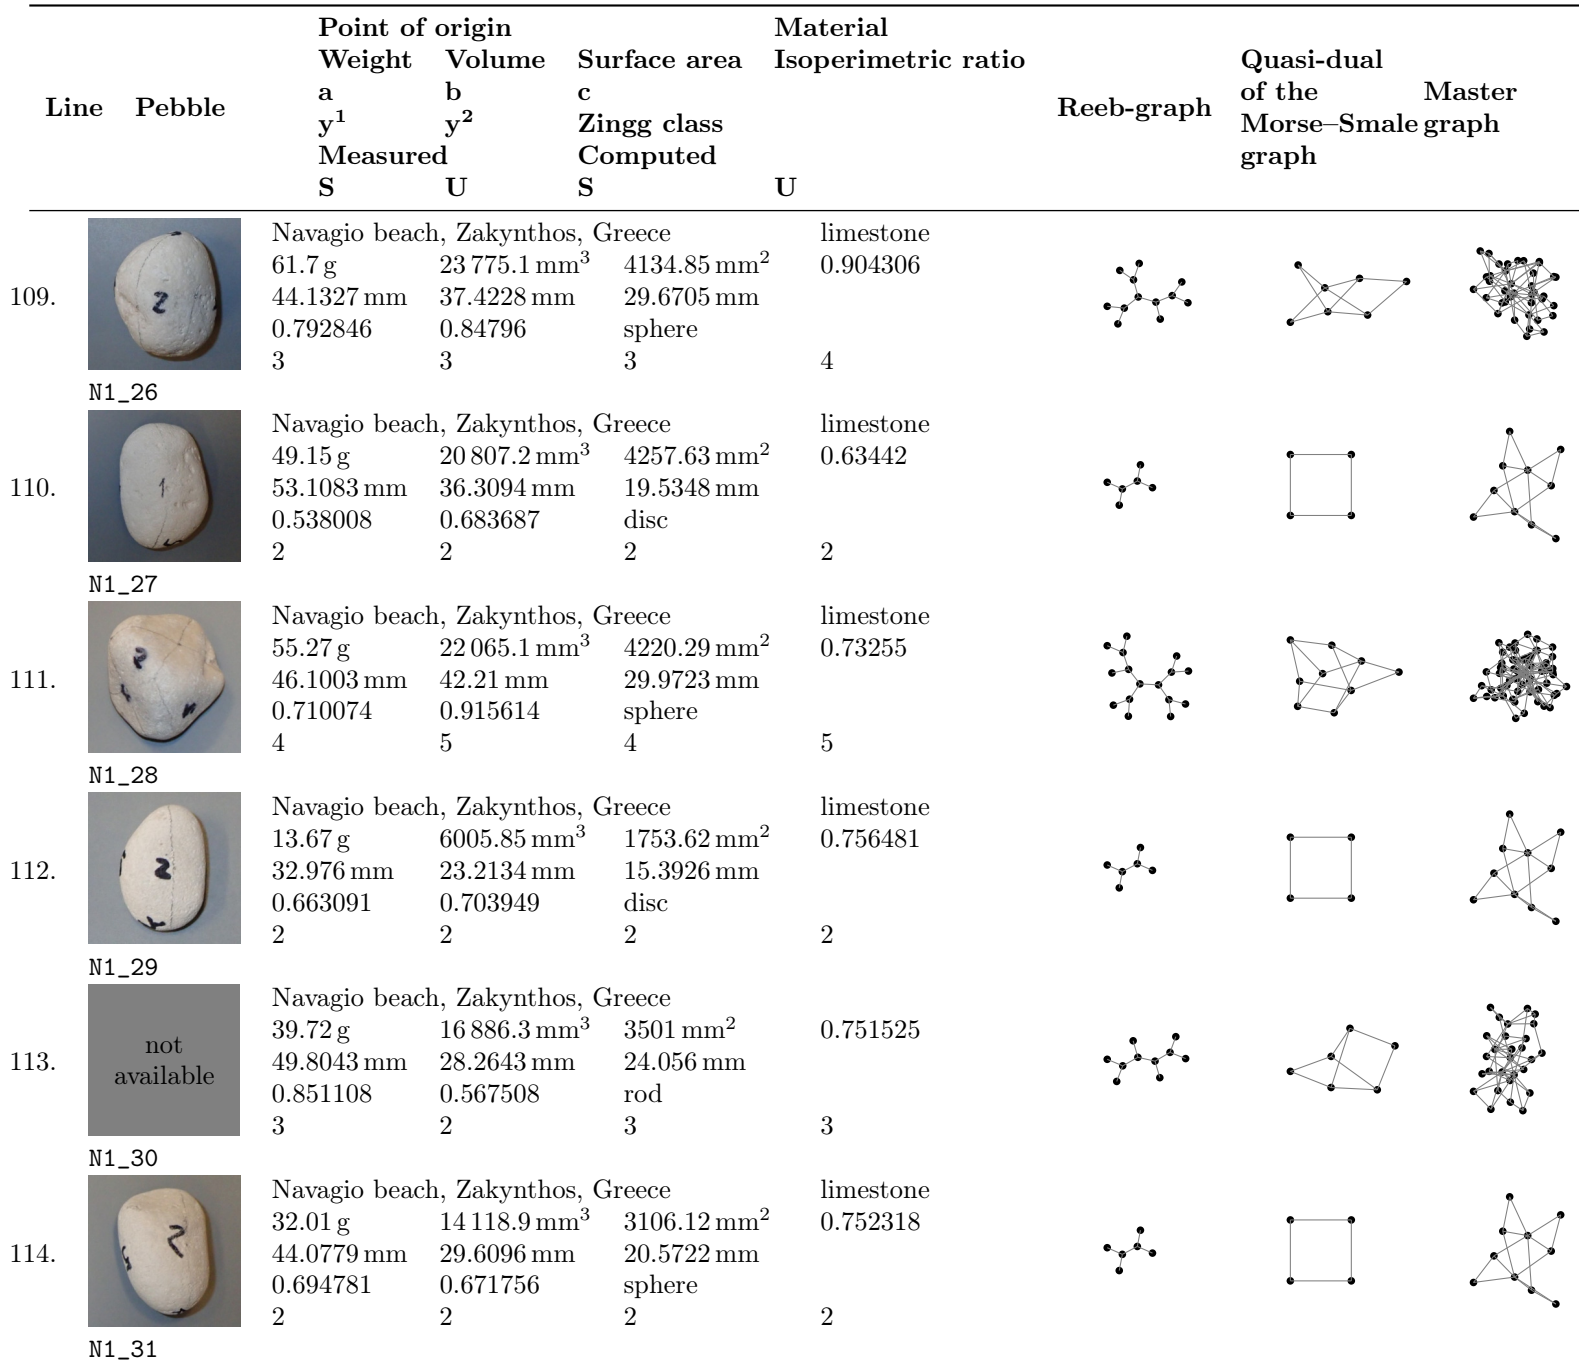 | Navagio beach, Zakynthos, Greece |                          |                         | limestone |                     |            |                                              |                 |
|      |                                                                                     | 32.01 g                          | 14 118.9 mm <sup>3</sup> | 3106.12 mm <sup>2</sup> | 0.752318  |                     |            |                                              |                 |
|      |                                                                                     | 44.0779 mm                       | 29.6096 mm               | 20.5722 mm              |           |                     |            |                                              |                 |
|      |                                                                                     | 0.694781                         | 0.671756                 | sphere                  |           |                     |            |                                              |                 |
|      |                                                                                     | 2                                | 2                        | 2                       | 2         |                     |            |                                              |                 |
|      |                                                                                     | N1_31                            |                          |                         |           |                     |            |                                              |                 |

| Line | Pebble                                                                              | Point of origin                                                            |                                                         |                                                    | Material                       | Reeb-graph                                                                            | Quasi-dual<br>of the<br>Morse–Smale<br>graph                                          | Master                                                                                |
|------|-------------------------------------------------------------------------------------|----------------------------------------------------------------------------|---------------------------------------------------------|----------------------------------------------------|--------------------------------|---------------------------------------------------------------------------------------|---------------------------------------------------------------------------------------|---------------------------------------------------------------------------------------|
|      |                                                                                     | Weight                                                                     | Volume                                                  | Surface area                                       |                                |                                                                                       |                                                                                       |                                                                                       |
|      |                                                                                     | a                                                                          | b                                                       | c                                                  |                                |                                                                                       |                                                                                       |                                                                                       |
|      |                                                                                     | y <sup>1</sup><br>Measured<br>S                                            | y <sup>2</sup><br>U                                     | Zingg class<br>Computed<br>S                       |                                |                                                                                       |                                                                                       |                                                                                       |
| 115. | 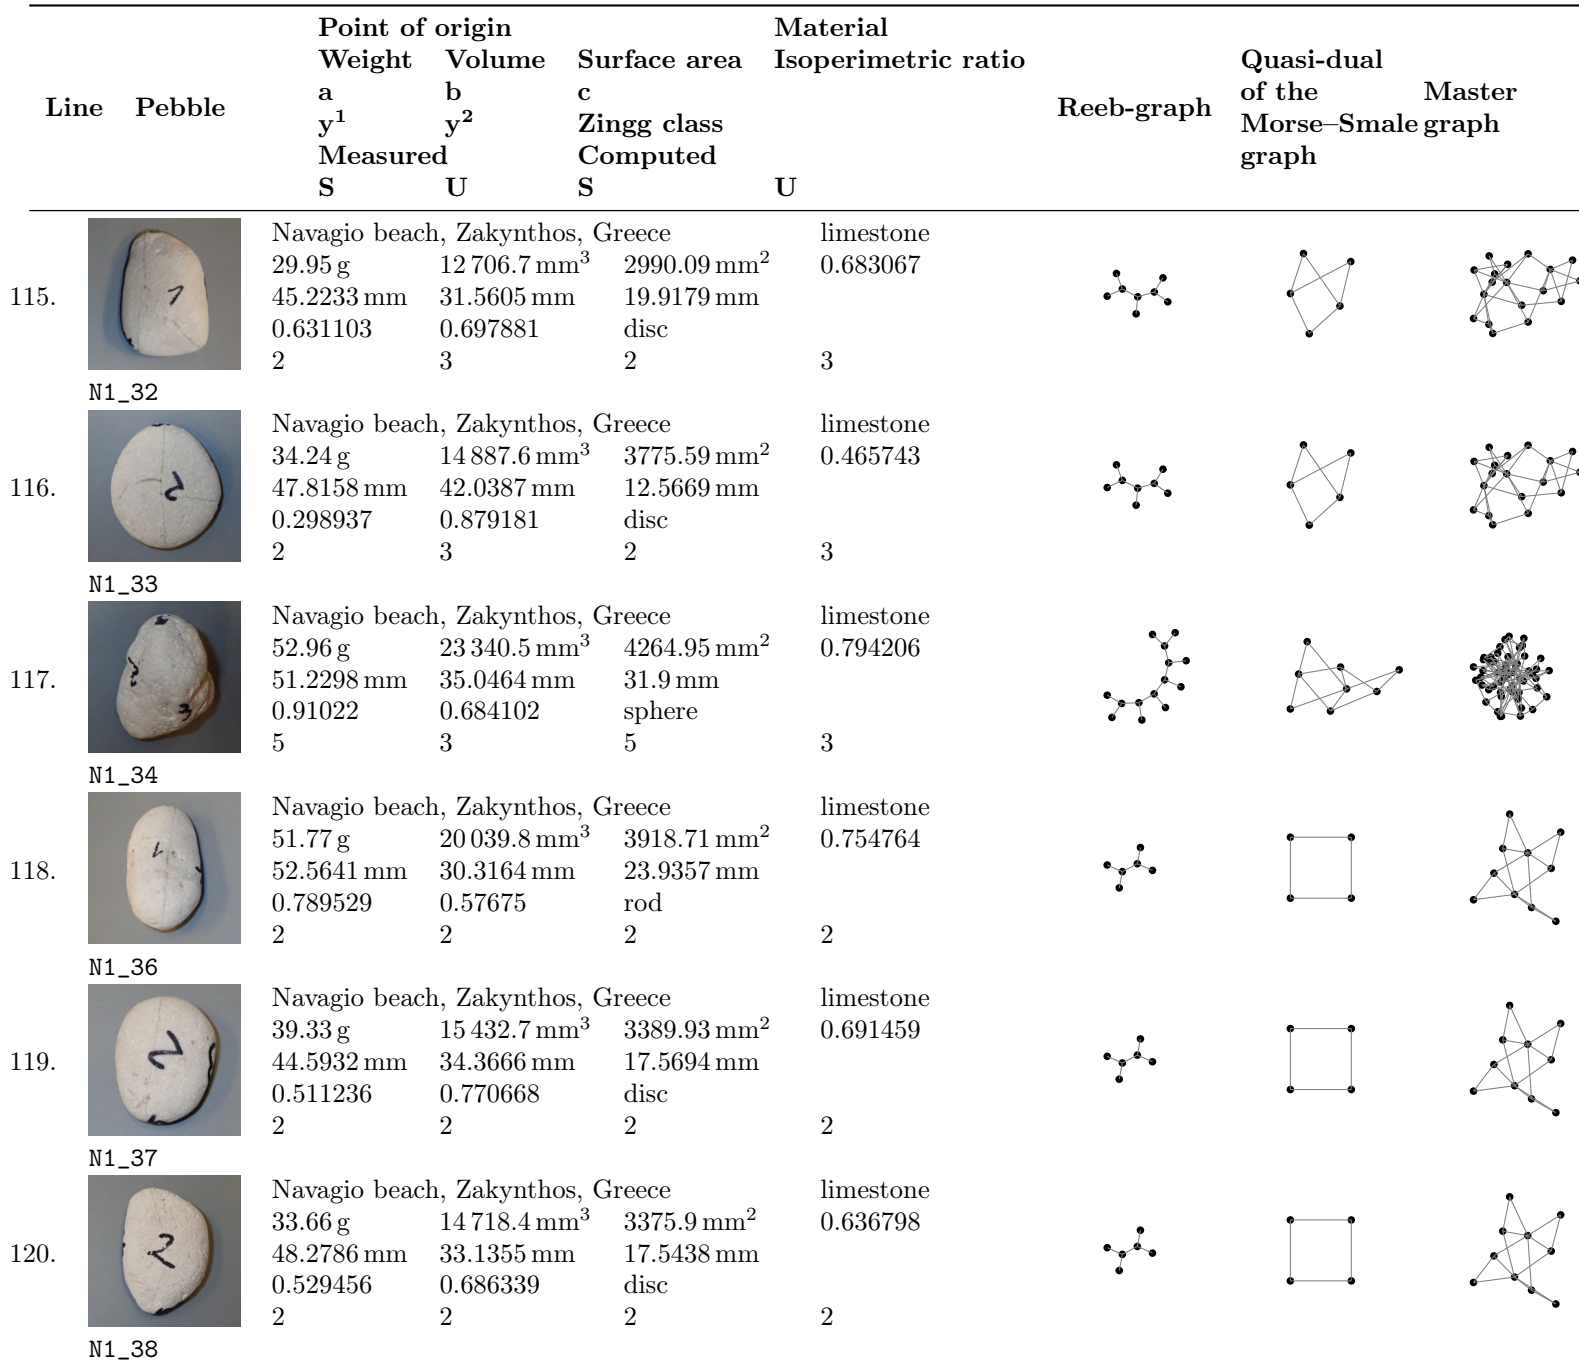   | Navagio beach, Zakynthos, Greece<br>29.95 g<br>45.2233 mm<br>0.631103<br>2 | 12 706.7 mm <sup>3</sup><br>31.5605 mm<br>0.697881<br>3 | 2990.09 mm <sup>2</sup><br>19.9179 mm<br>disc<br>2 | limestone<br>0.683067<br><br>3 | 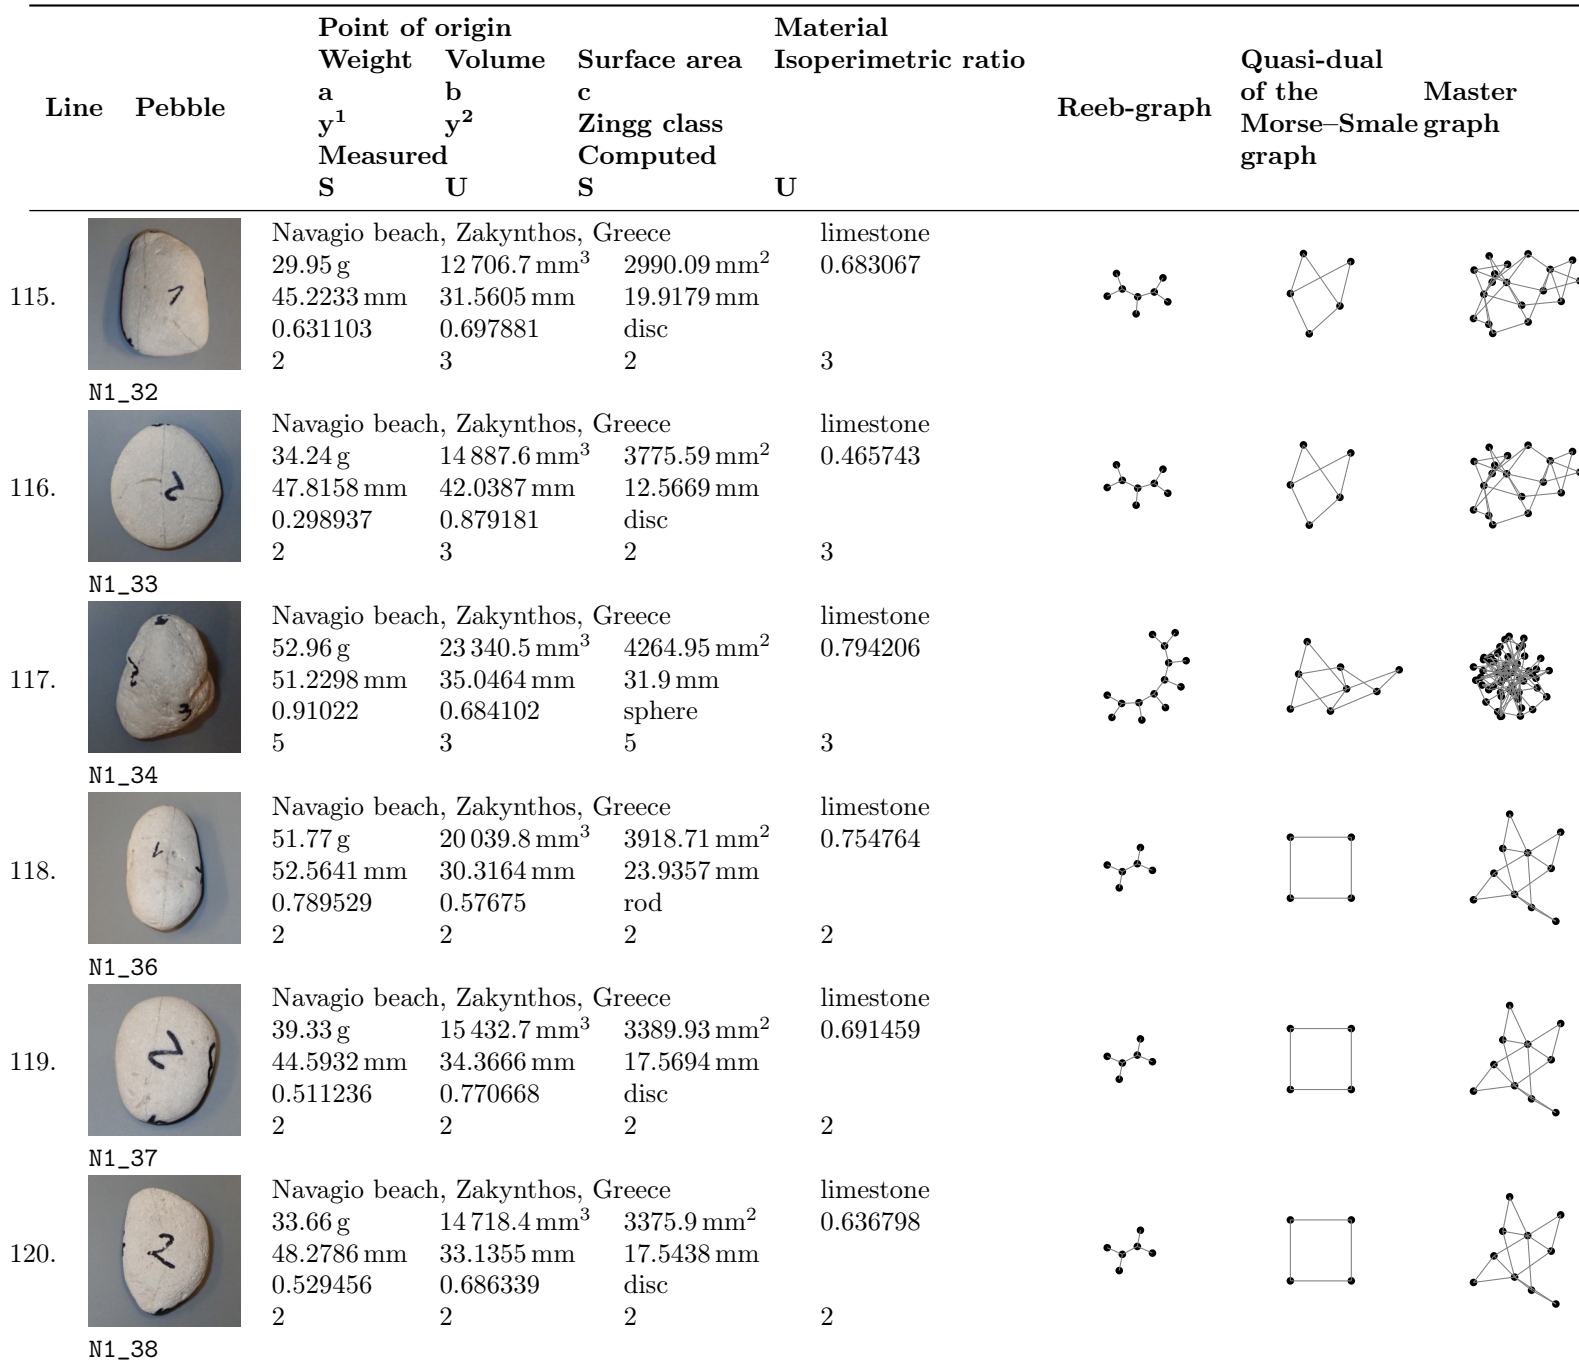   | 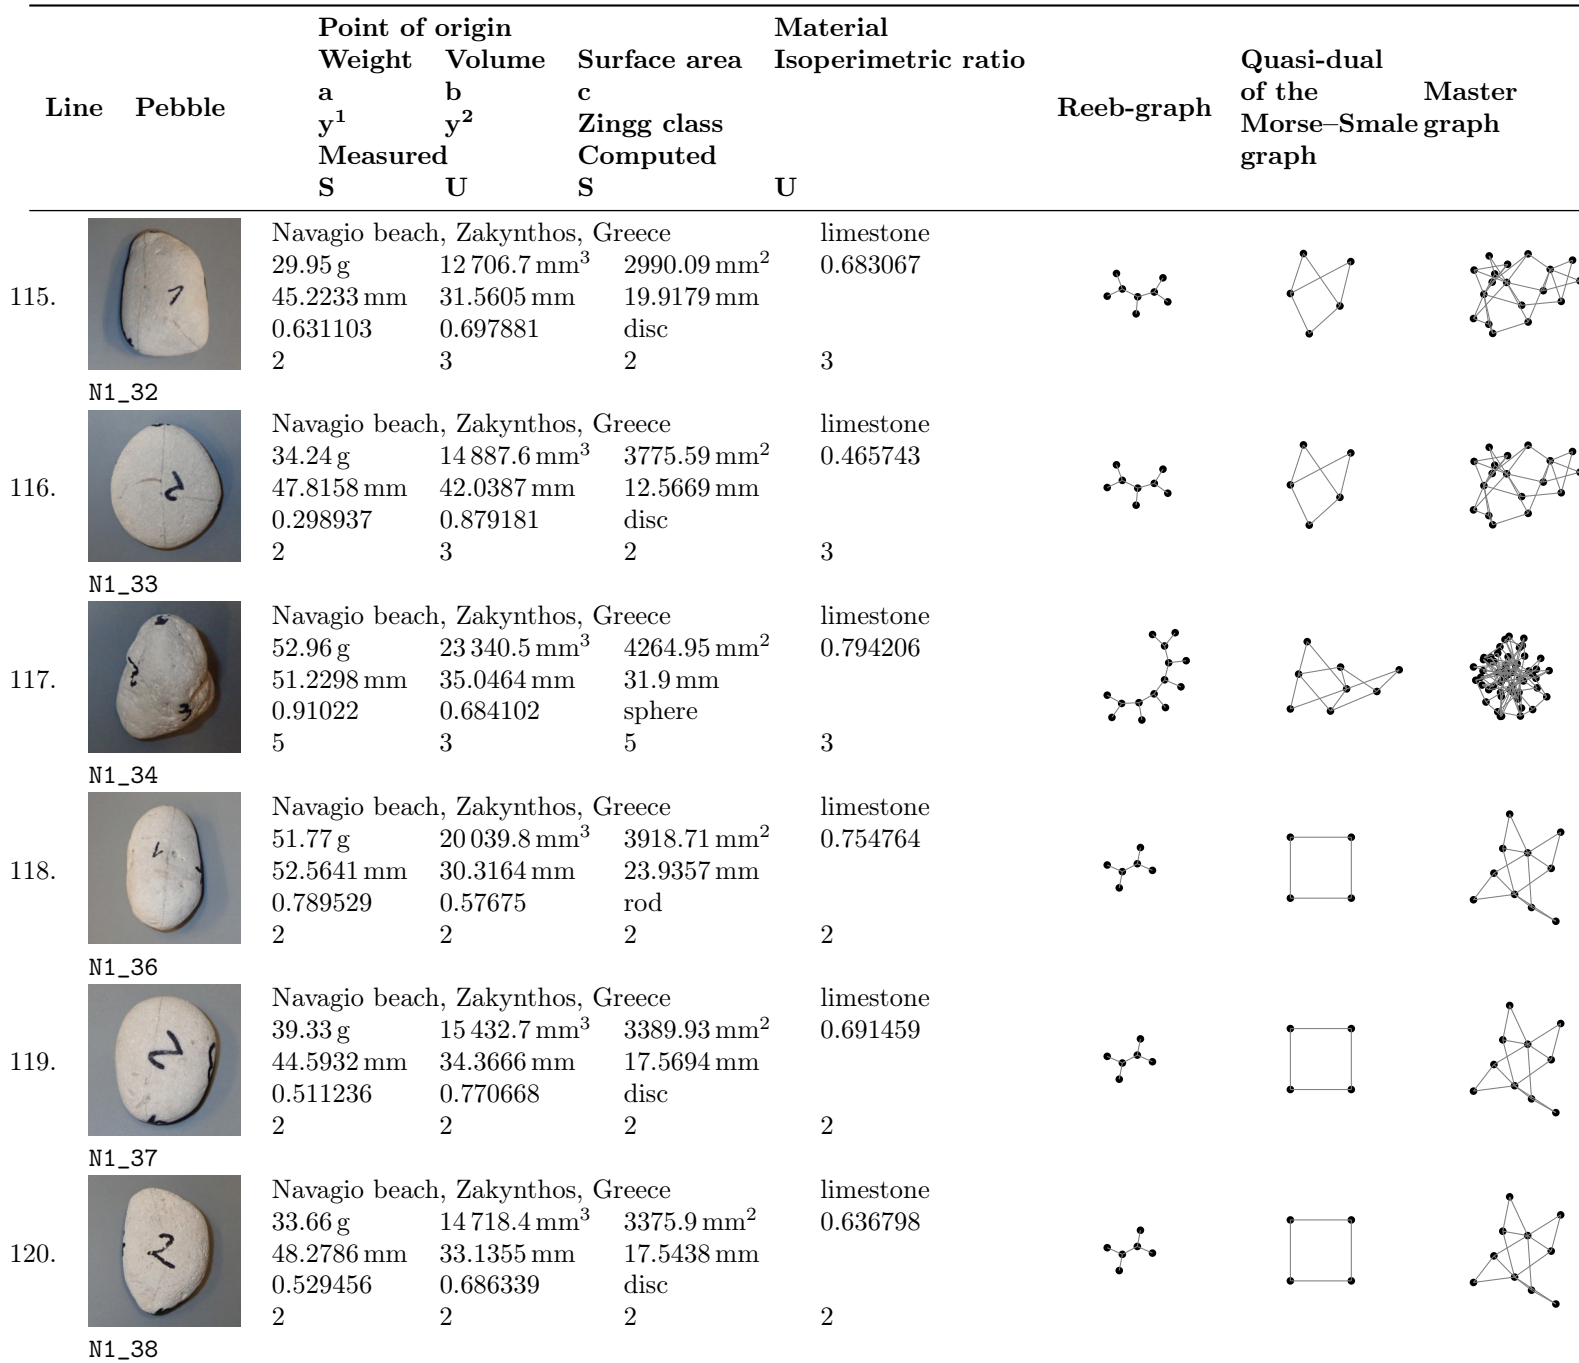   | 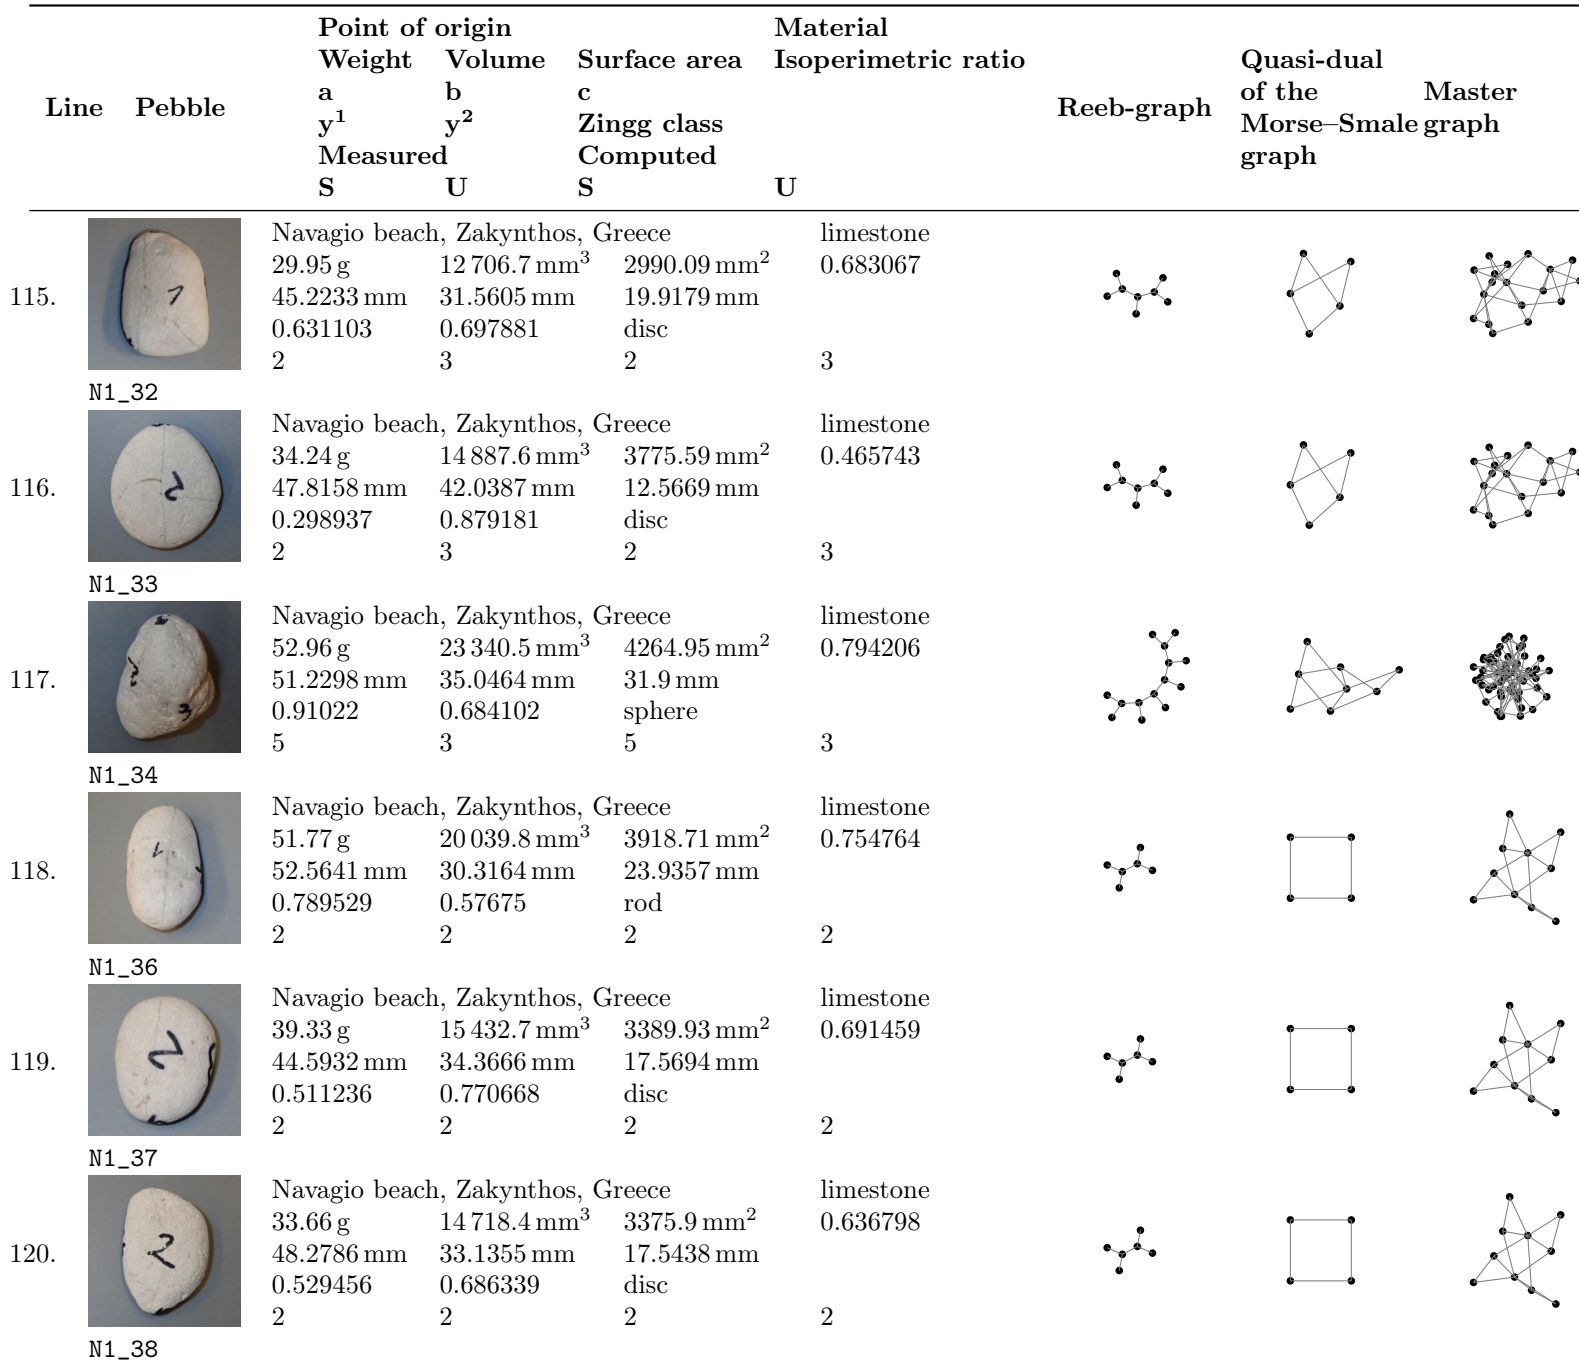   |
|      | N1_32                                                                               |                                                                            |                                                         |                                                    |                                |                                                                                       |                                                                                       |                                                                                       |
| 116. | 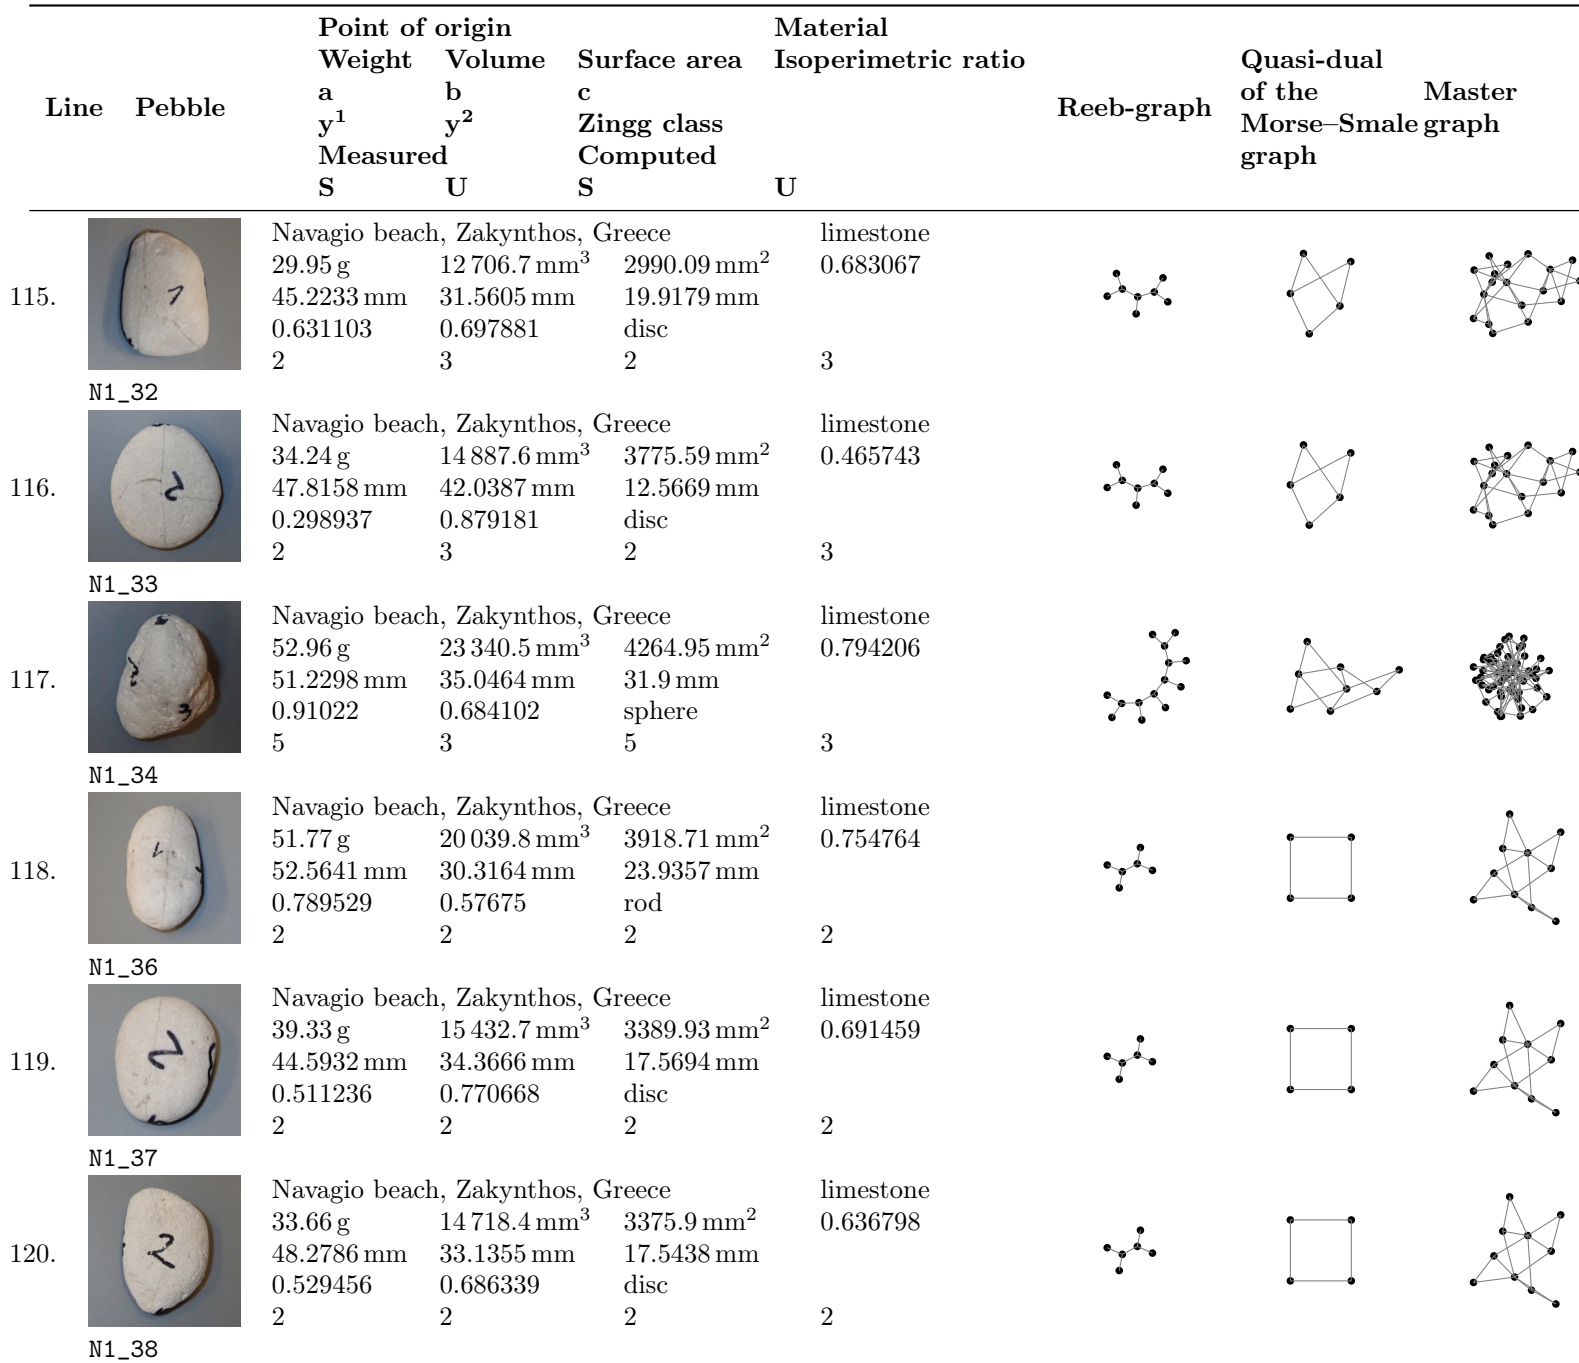   | Navagio beach, Zakynthos, Greece<br>34.24 g<br>47.8158 mm<br>0.298937<br>2 | 14 887.6 mm <sup>3</sup><br>42.0387 mm<br>0.879181<br>3 | 3775.59 mm <sup>2</sup><br>12.5669 mm<br>disc<br>2 | limestone<br>0.465743<br><br>3 | 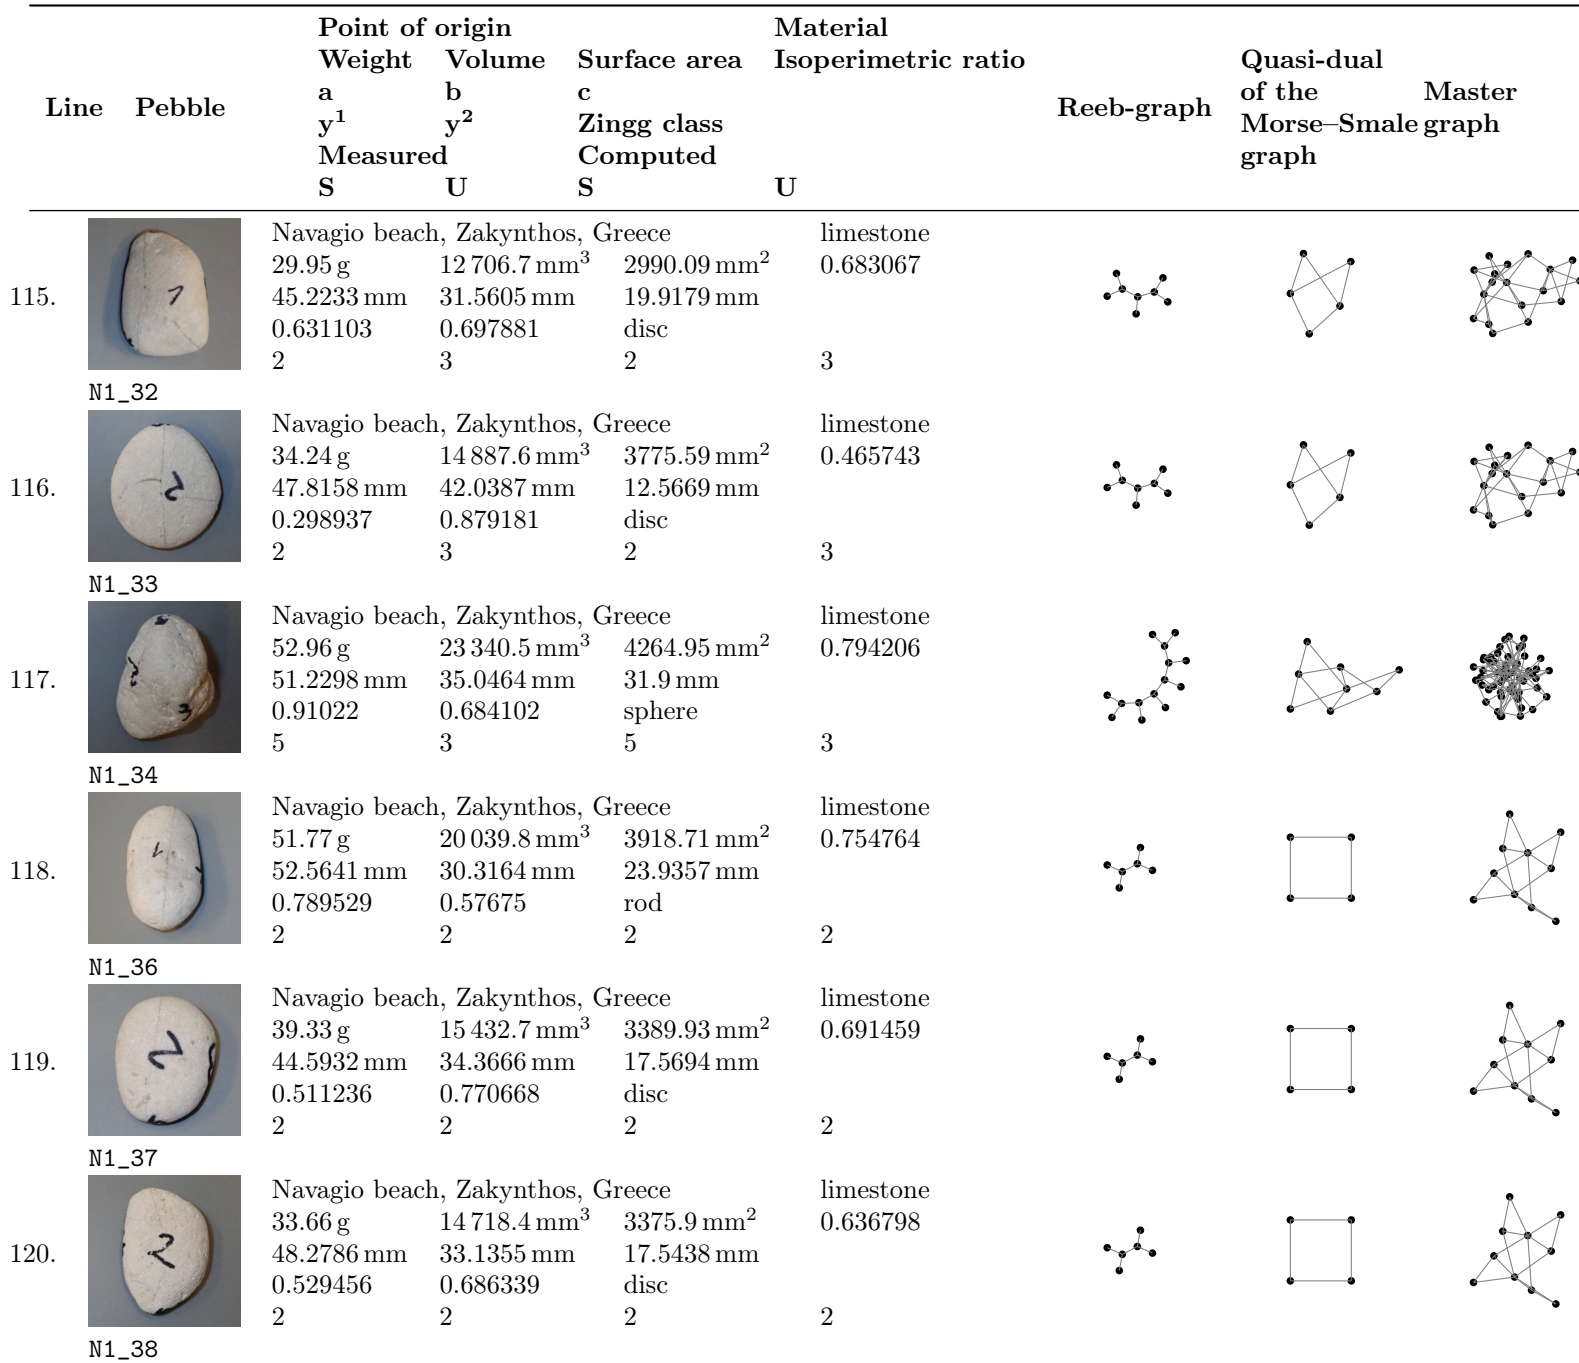   | 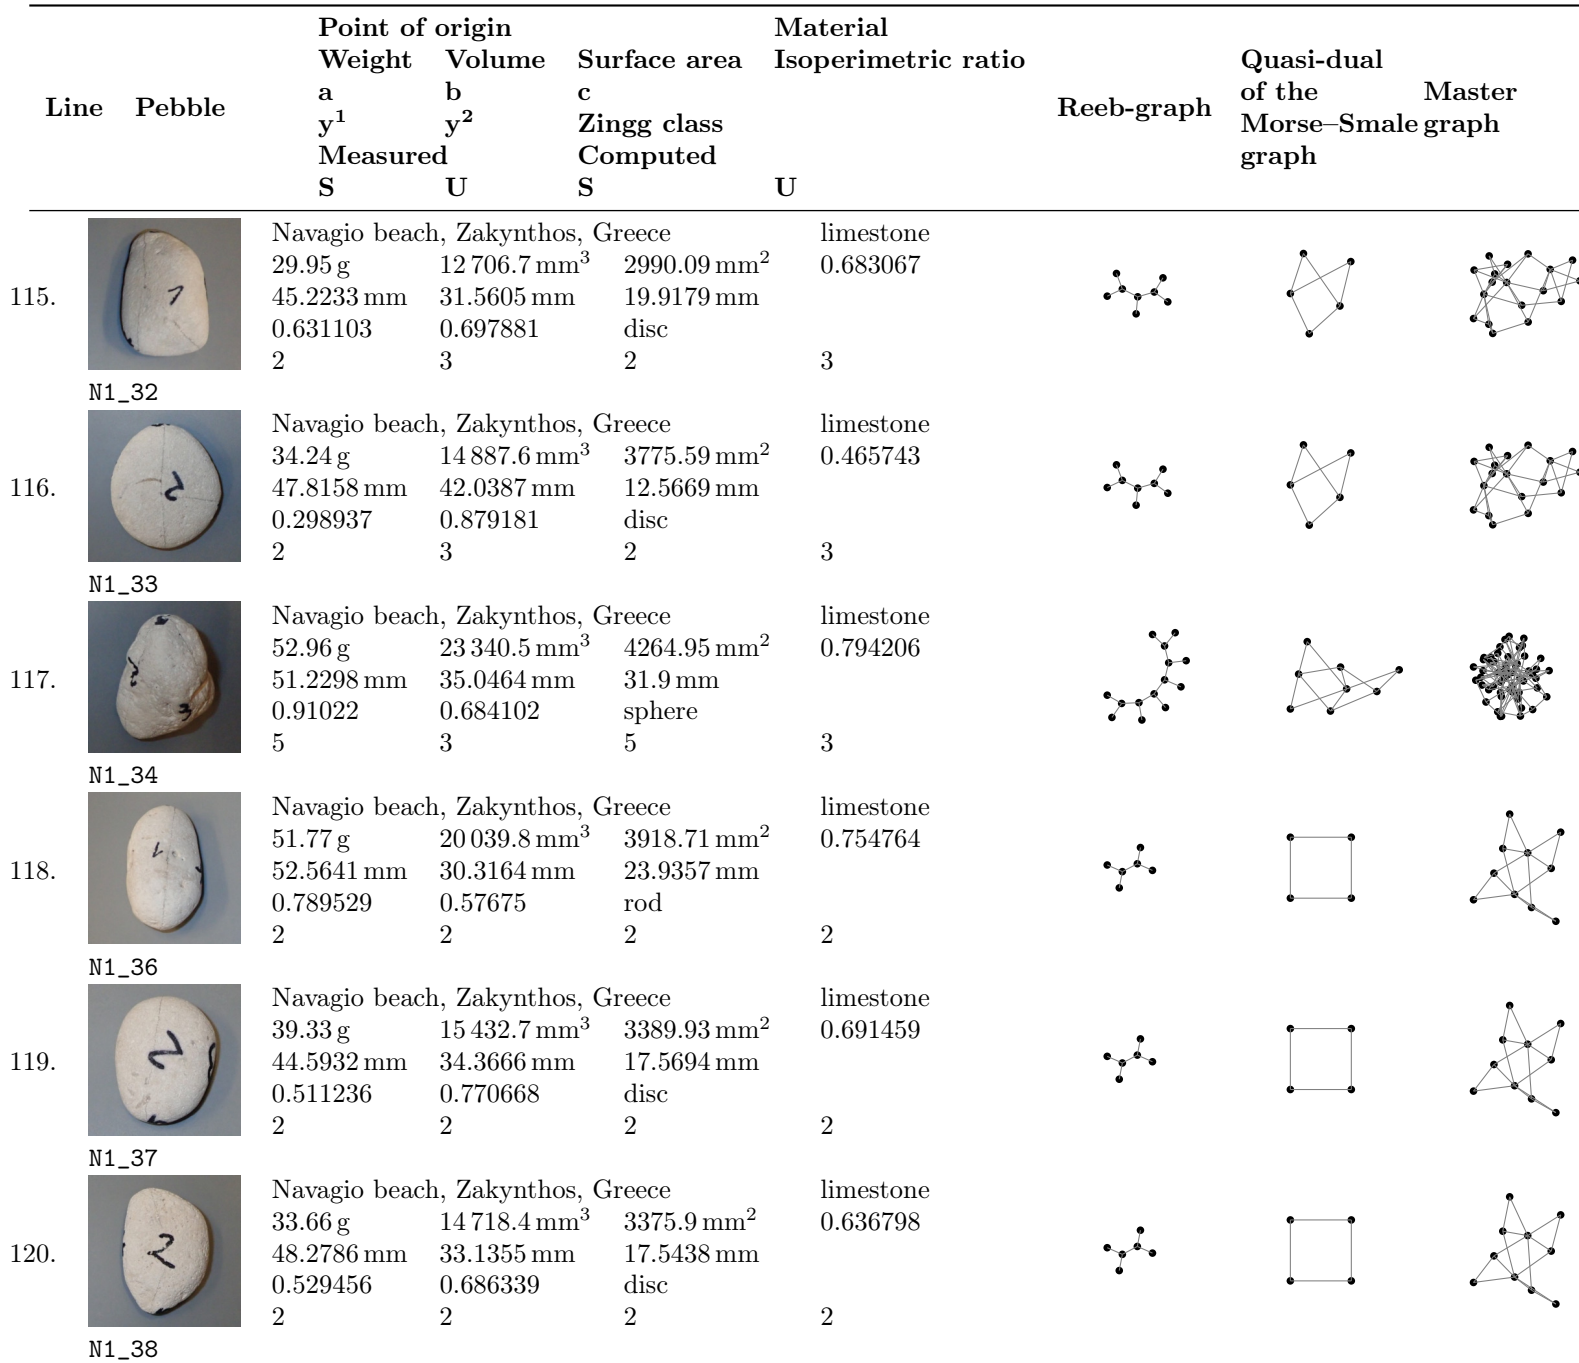   | 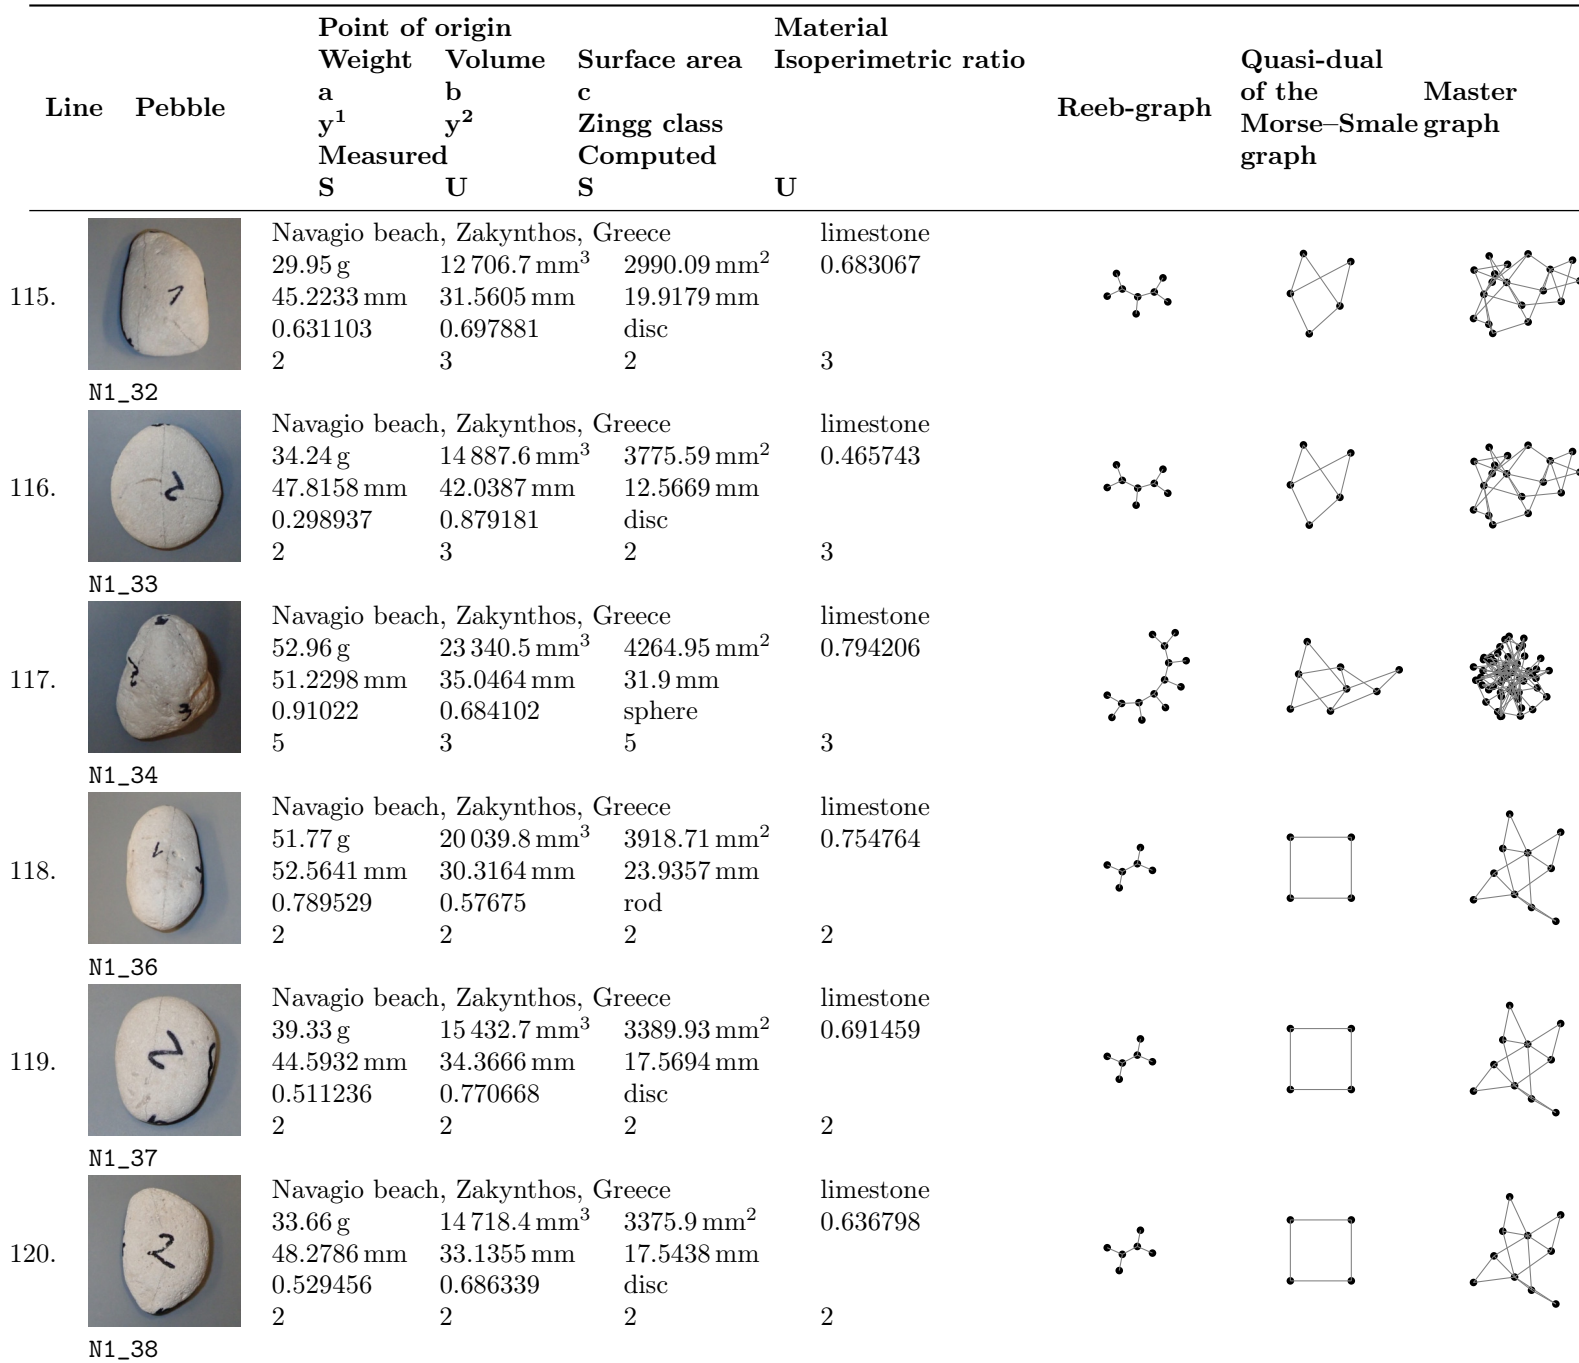   |
|      | N1_33                                                                               |                                                                            |                                                         |                                                    |                                |                                                                                       |                                                                                       |                                                                                       |
| 117. | 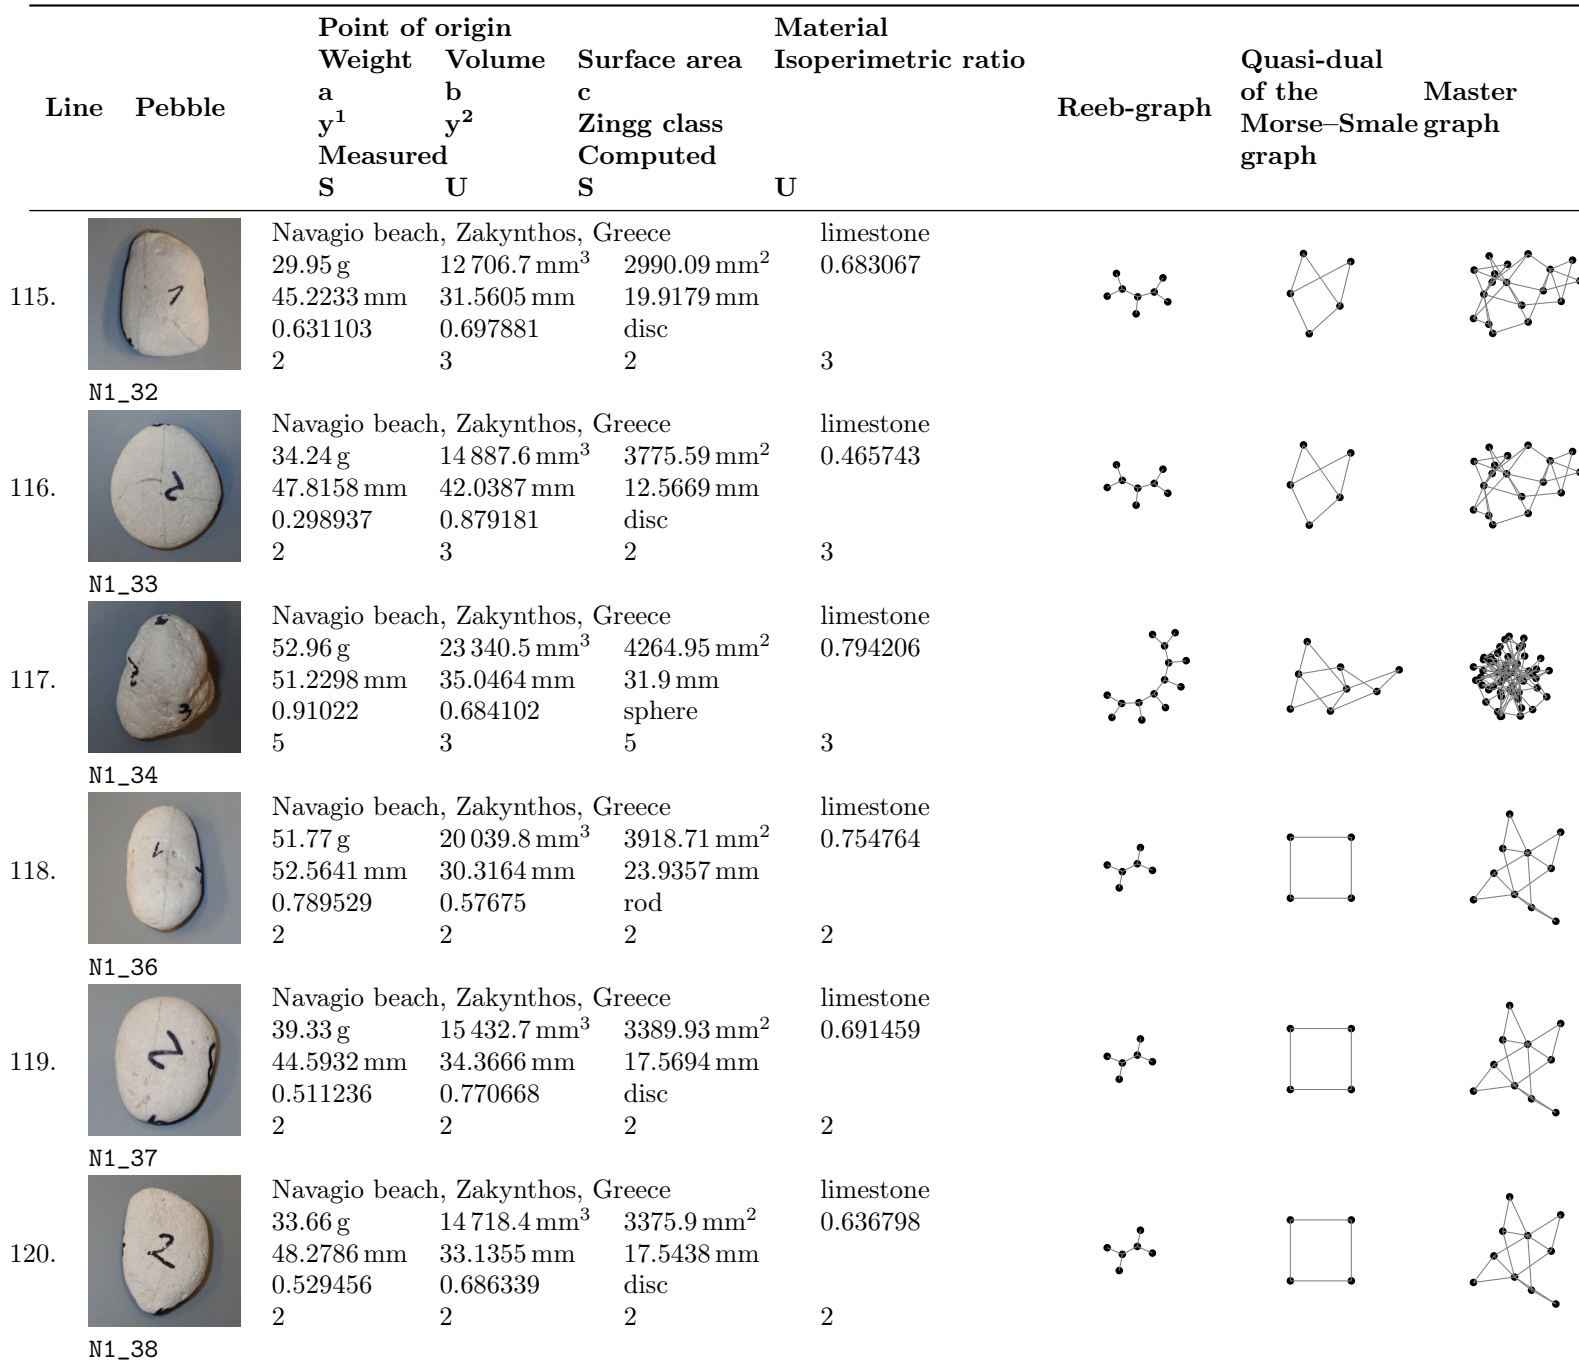   | Navagio beach, Zakynthos, Greece<br>52.96 g<br>51.2298 mm<br>0.91022<br>5  | 23 340.5 mm <sup>3</sup><br>35.0464 mm<br>0.684102<br>3 | 4264.95 mm <sup>2</sup><br>31.9 mm<br>sphere<br>5  | limestone<br>0.794206<br><br>3 | 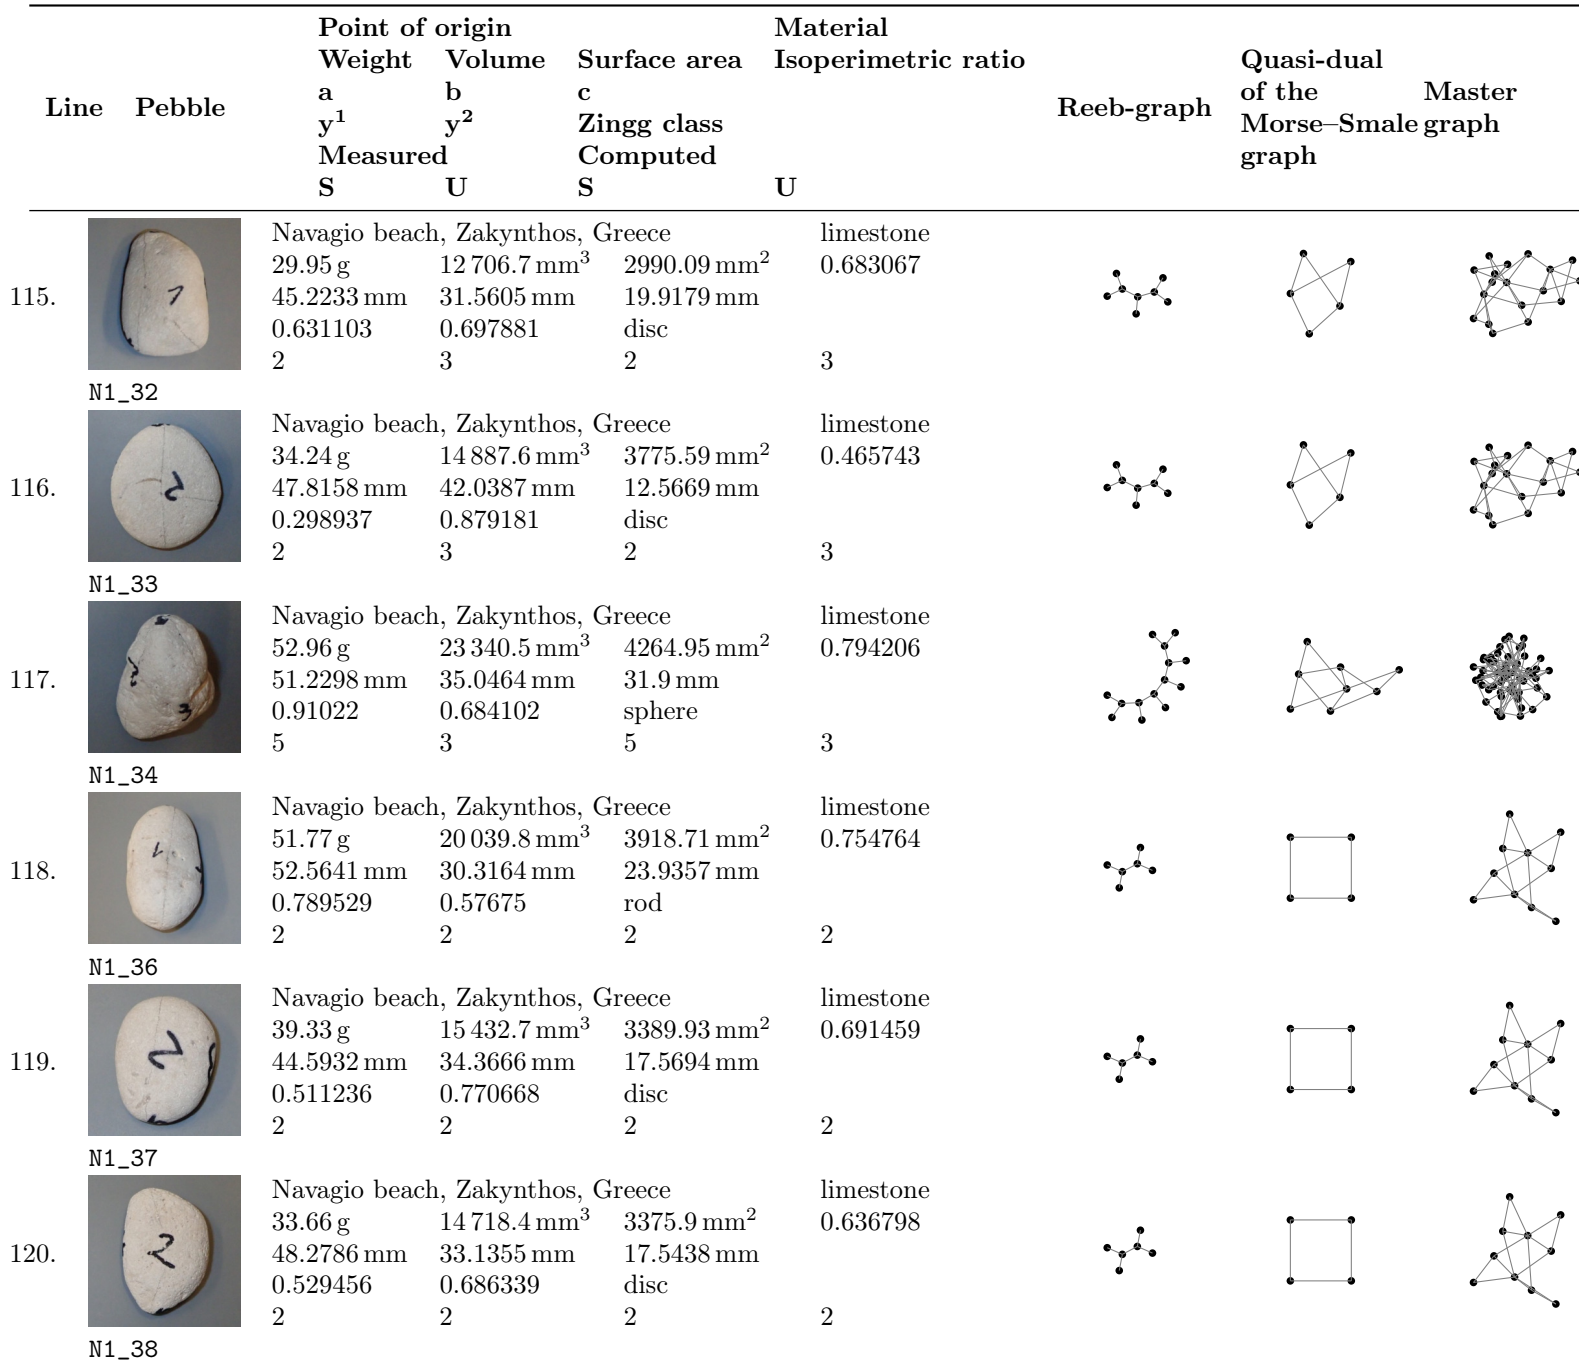   | 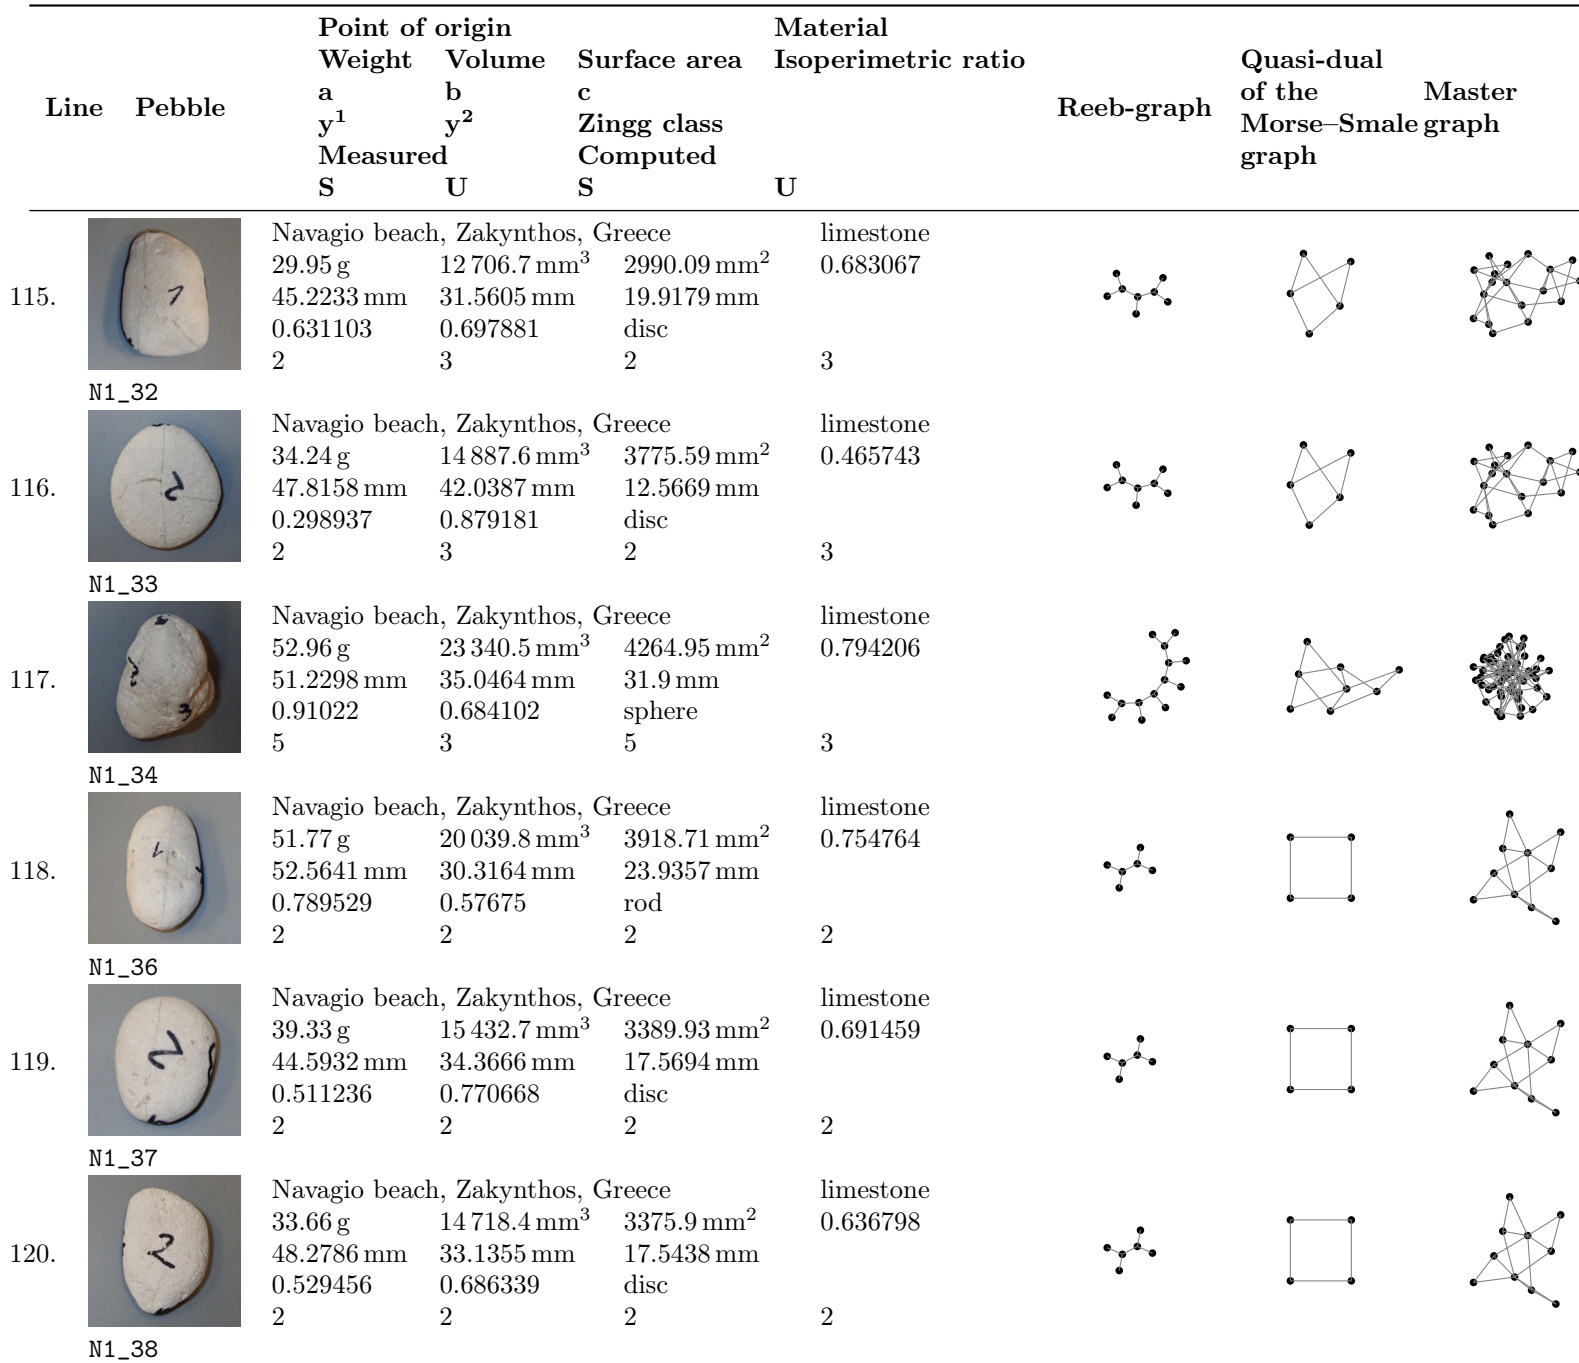   | 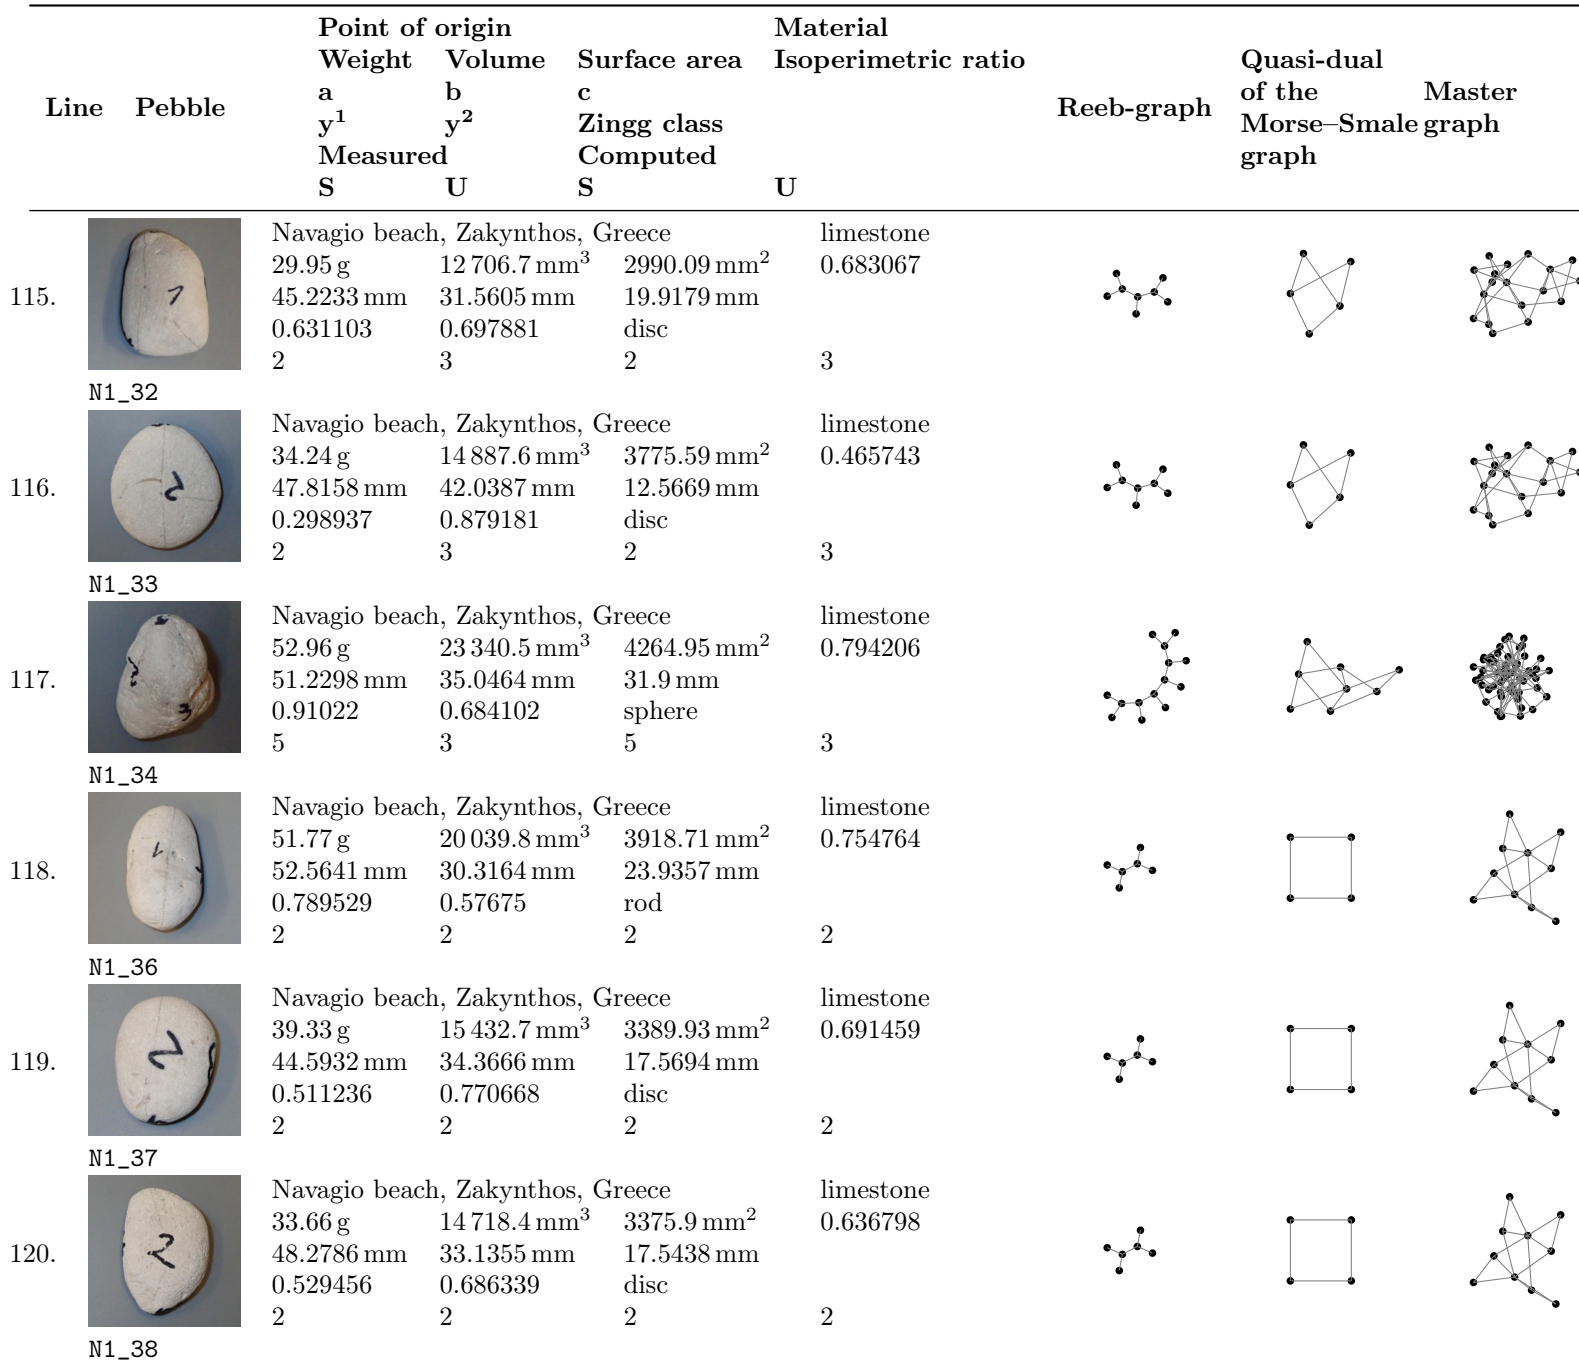   |
|      | N1_34                                                                               |                                                                            |                                                         |                                                    |                                |                                                                                       |                                                                                       |                                                                                       |
| 118. | 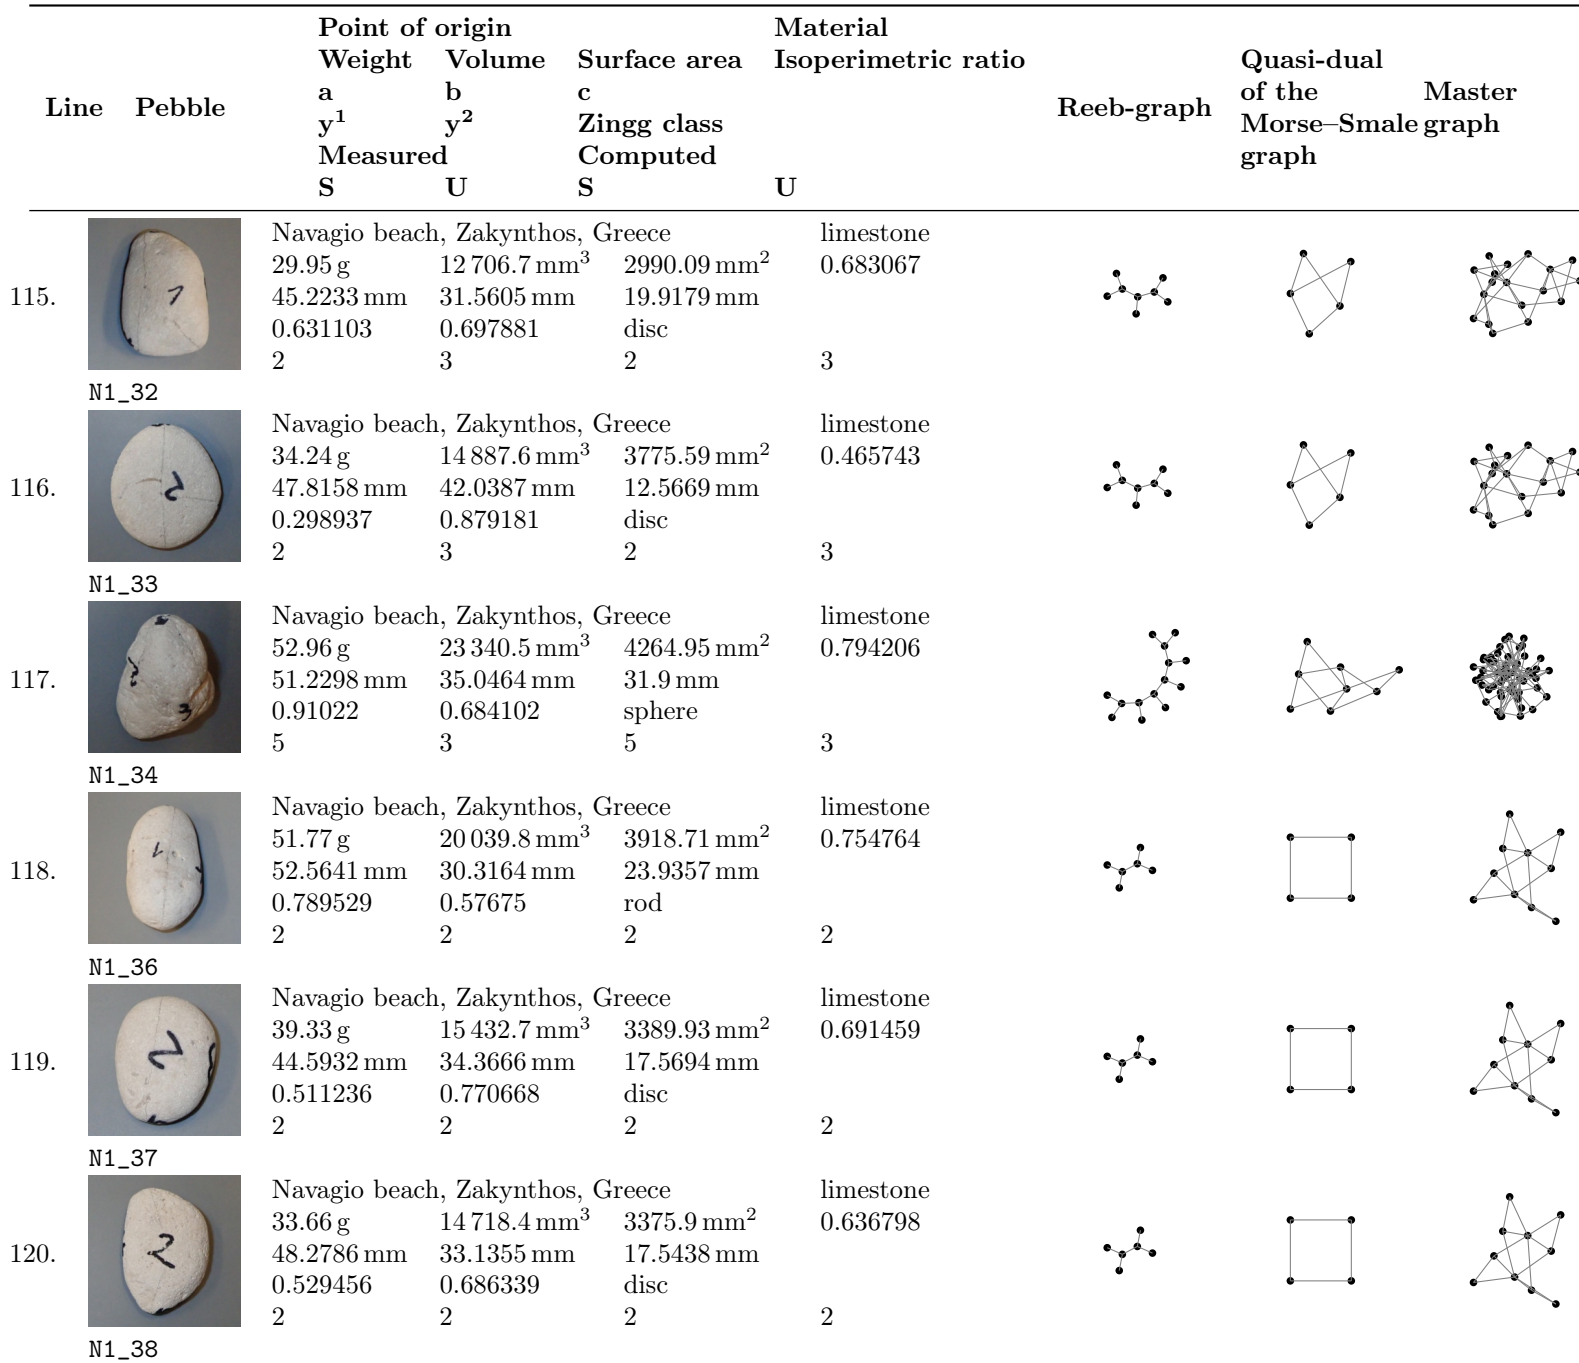  | Navagio beach, Zakynthos, Greece<br>51.77 g<br>52.5641 mm<br>0.789529<br>2 | 20 039.8 mm <sup>3</sup><br>30.3164 mm<br>0.57675<br>2  | 3918.71 mm <sup>2</sup><br>23.9357 mm<br>rod<br>2  | limestone<br>0.754764<br><br>2 | 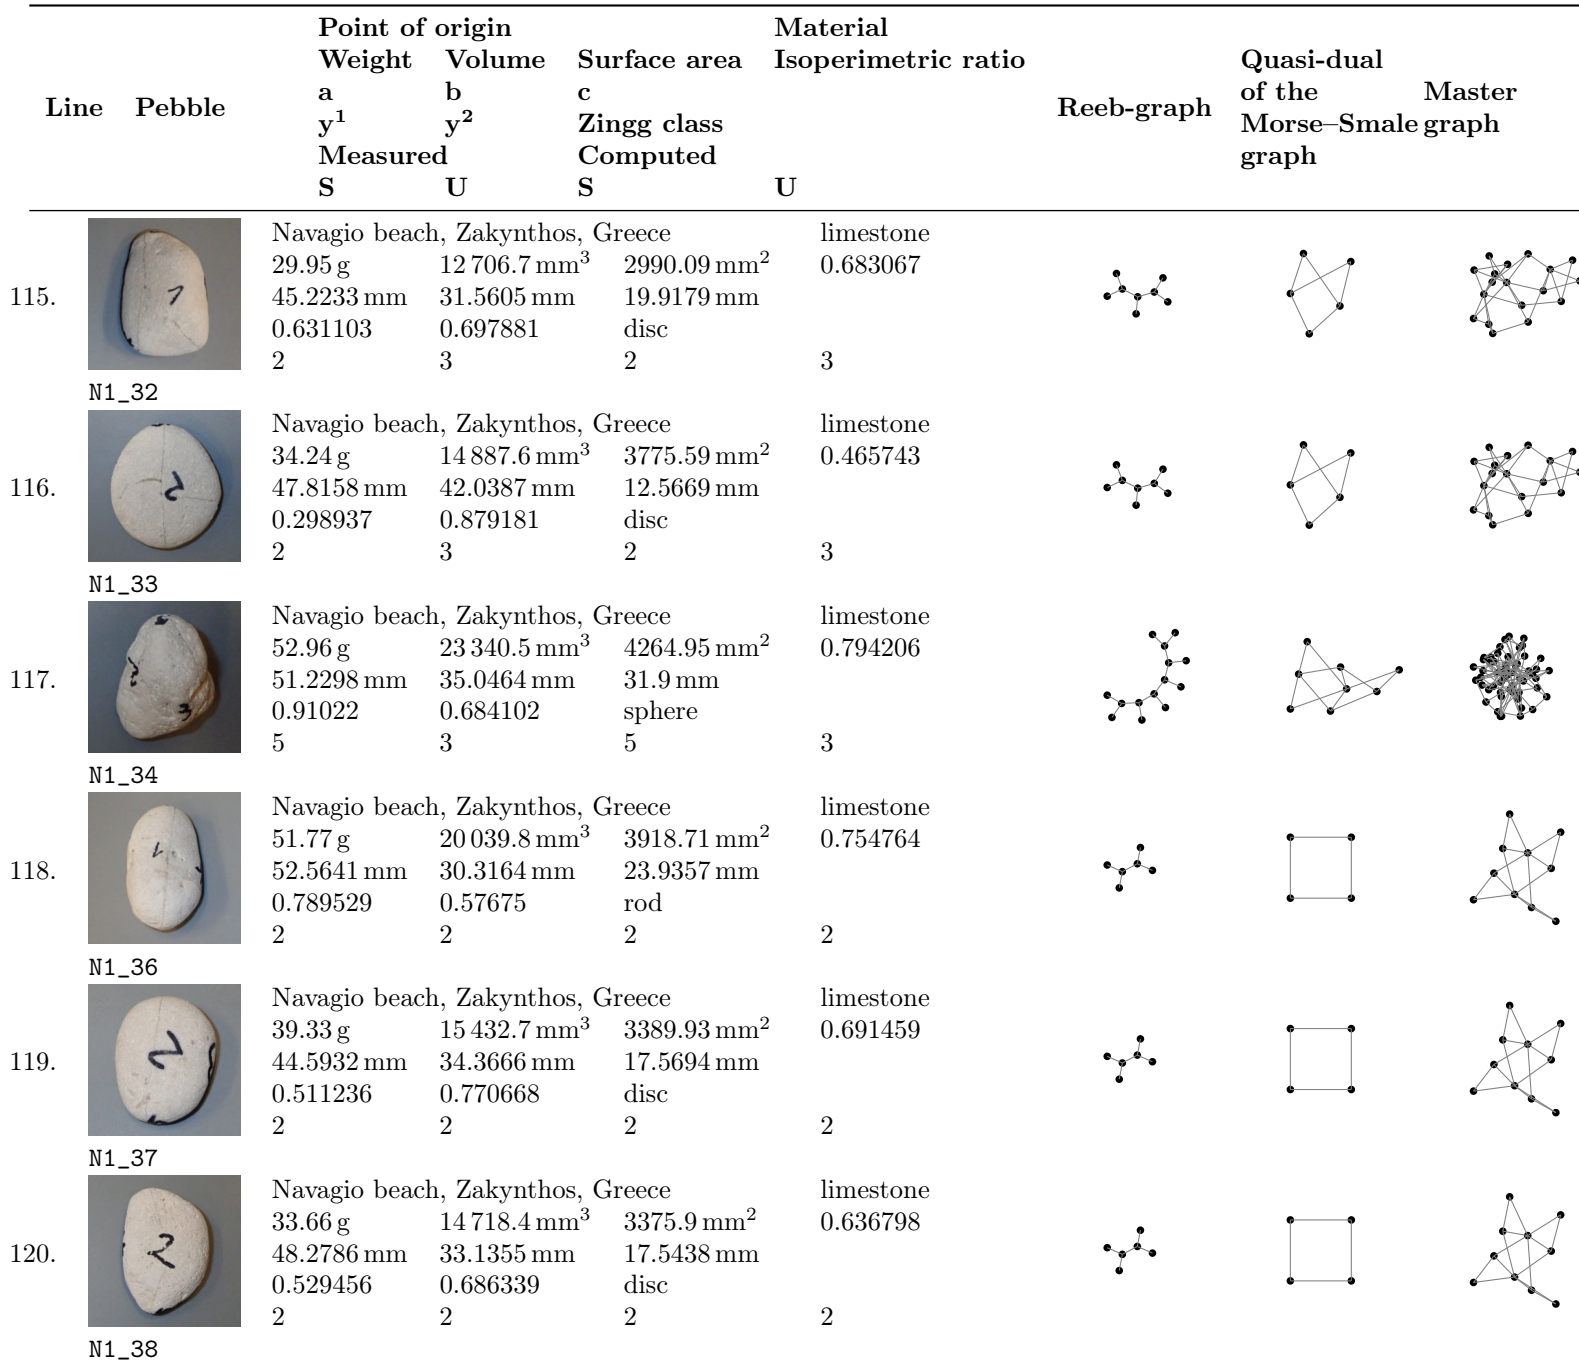  | 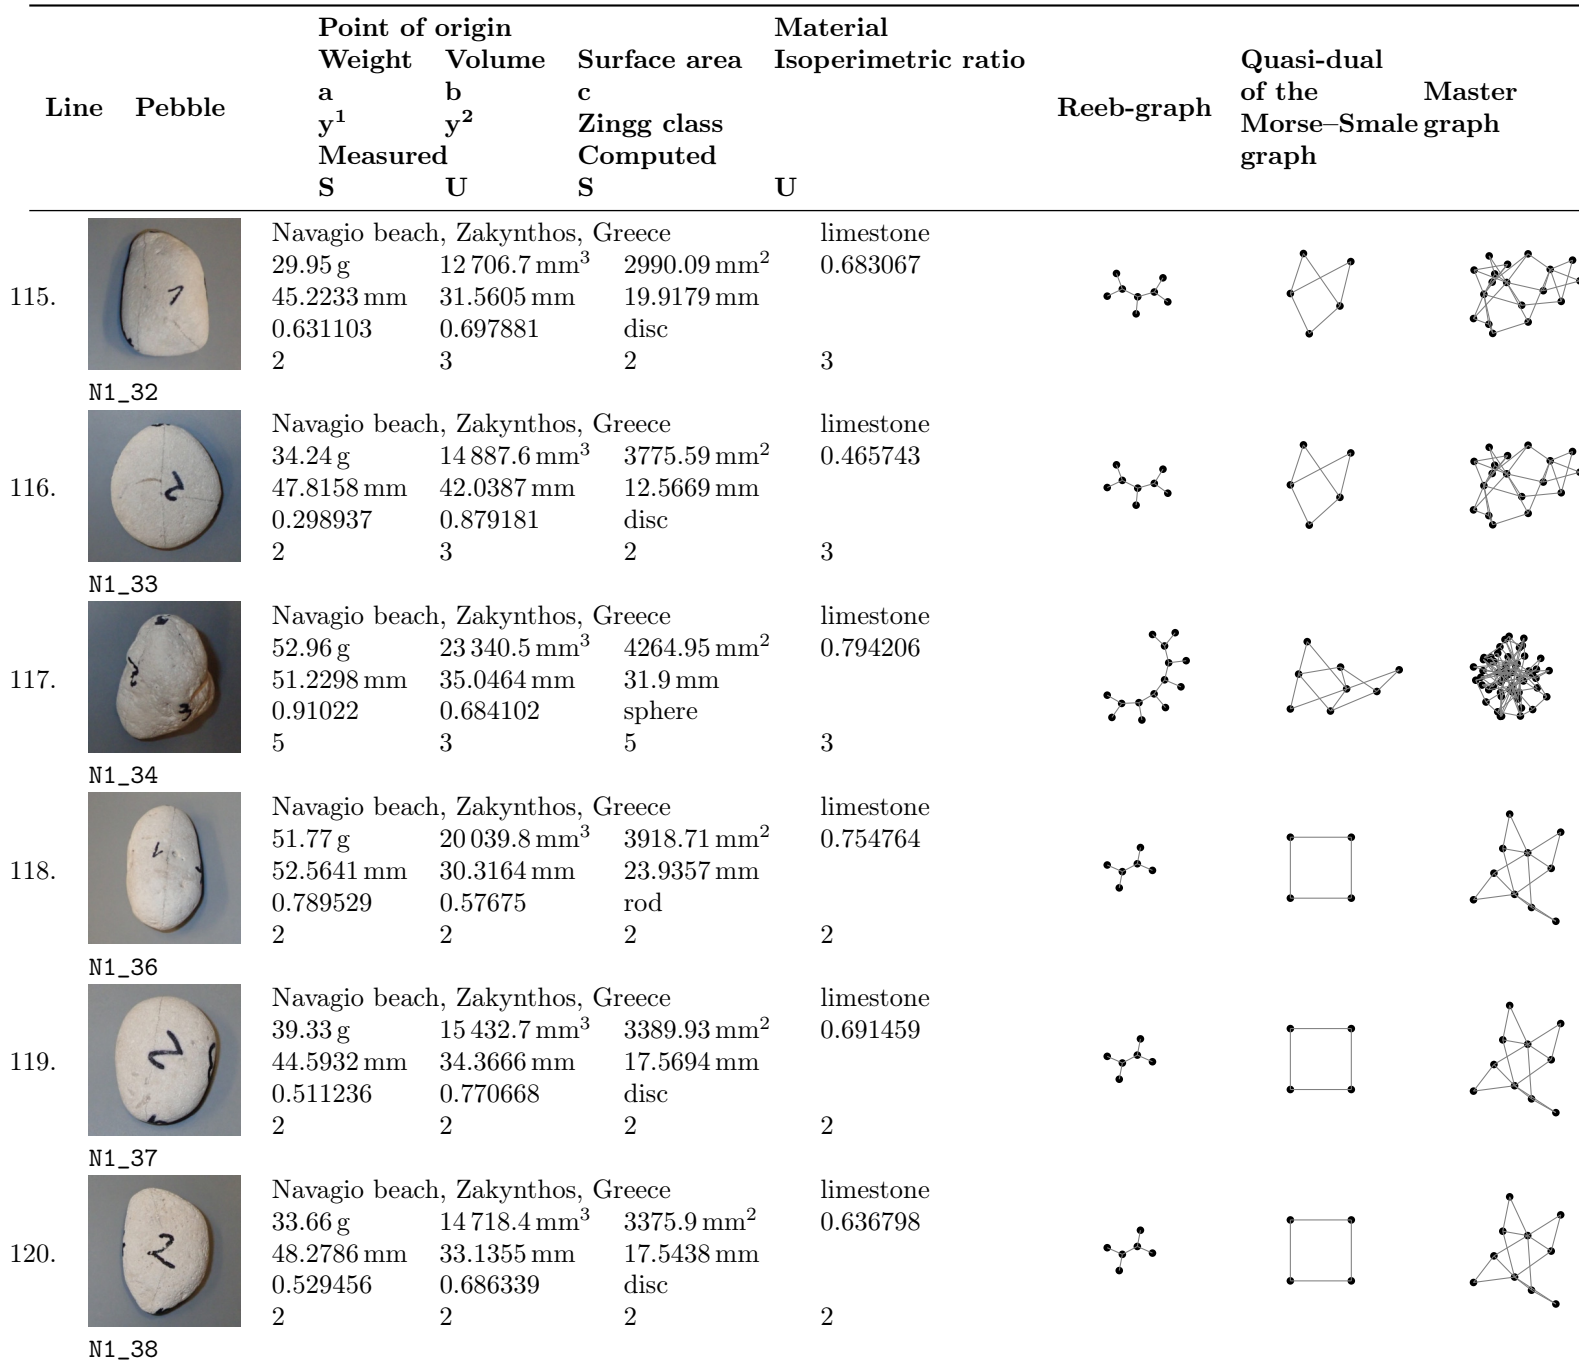  | 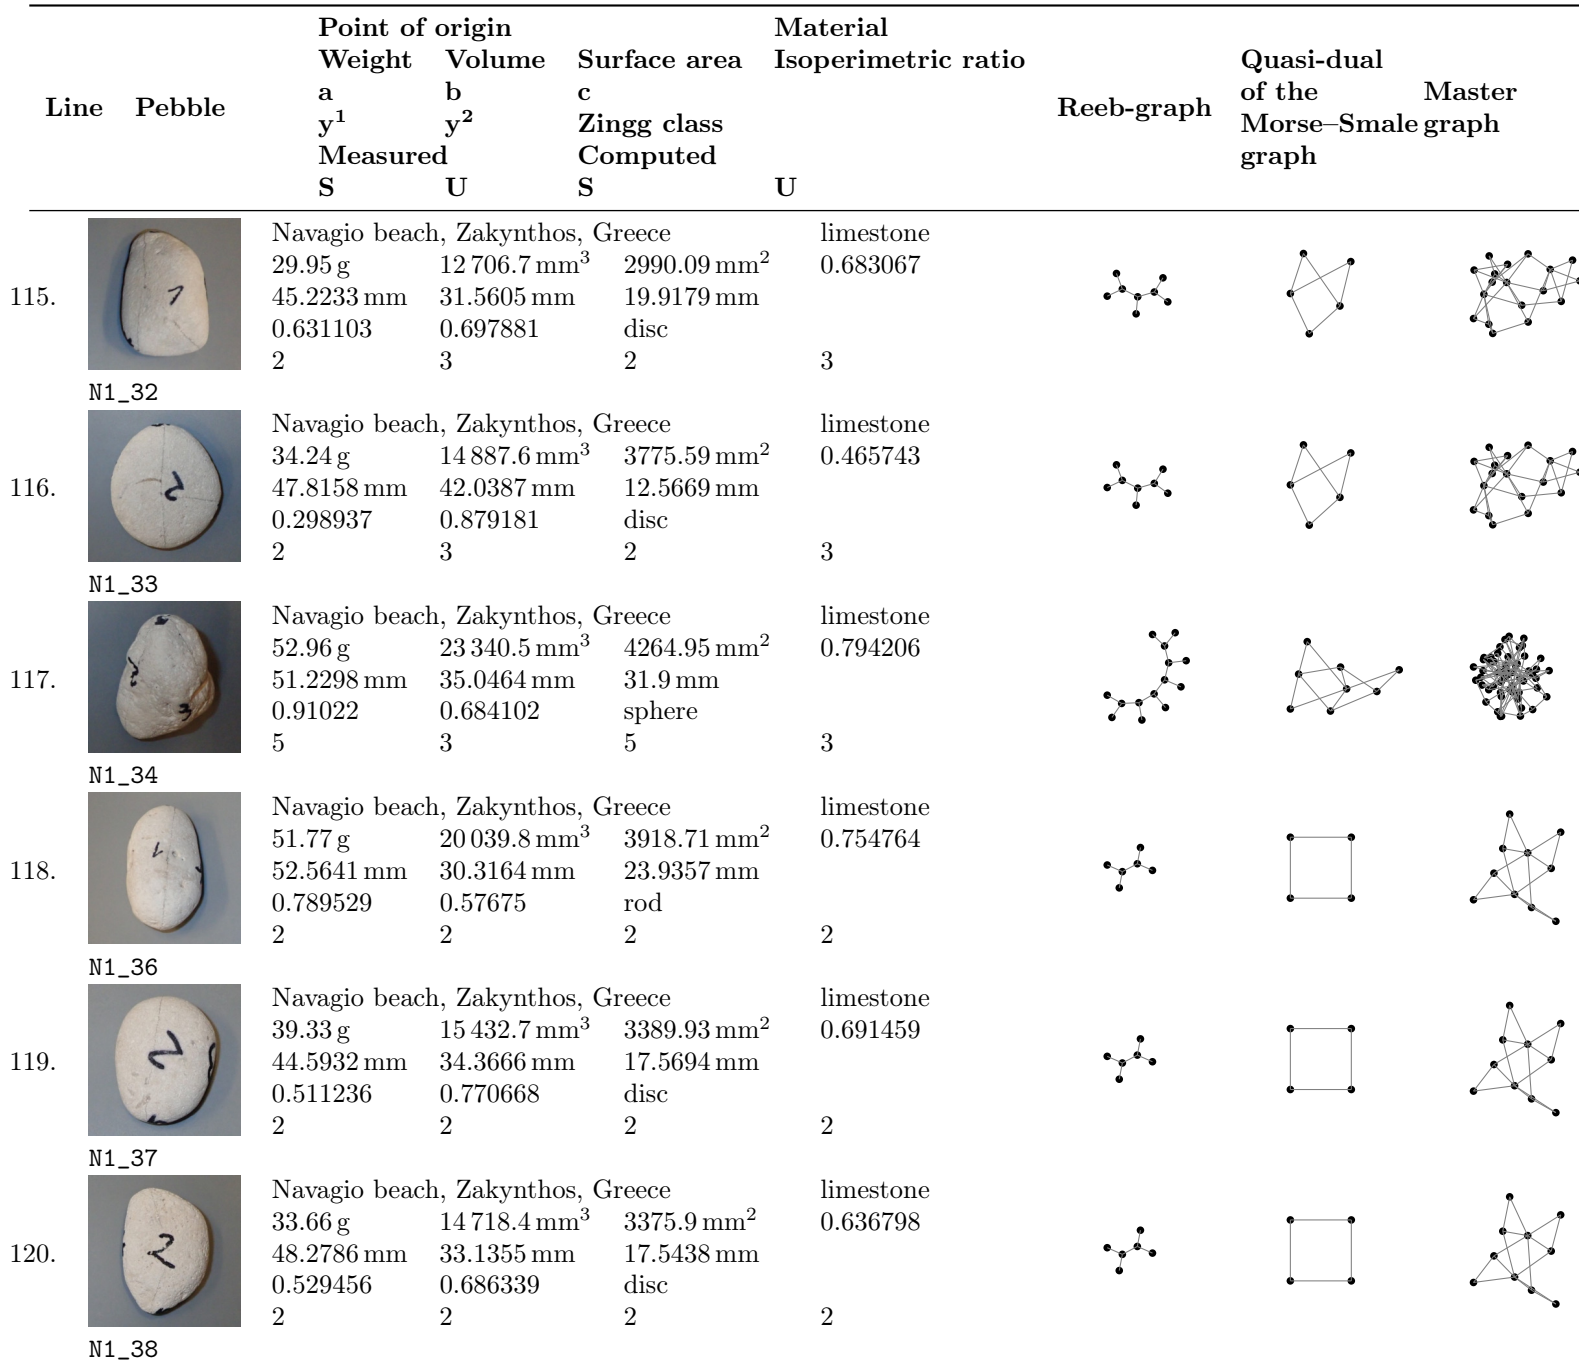  |
|      | N1_36                                                                               |                                                                            |                                                         |                                                    |                                |                                                                                       |                                                                                       |                                                                                       |
| 119. | 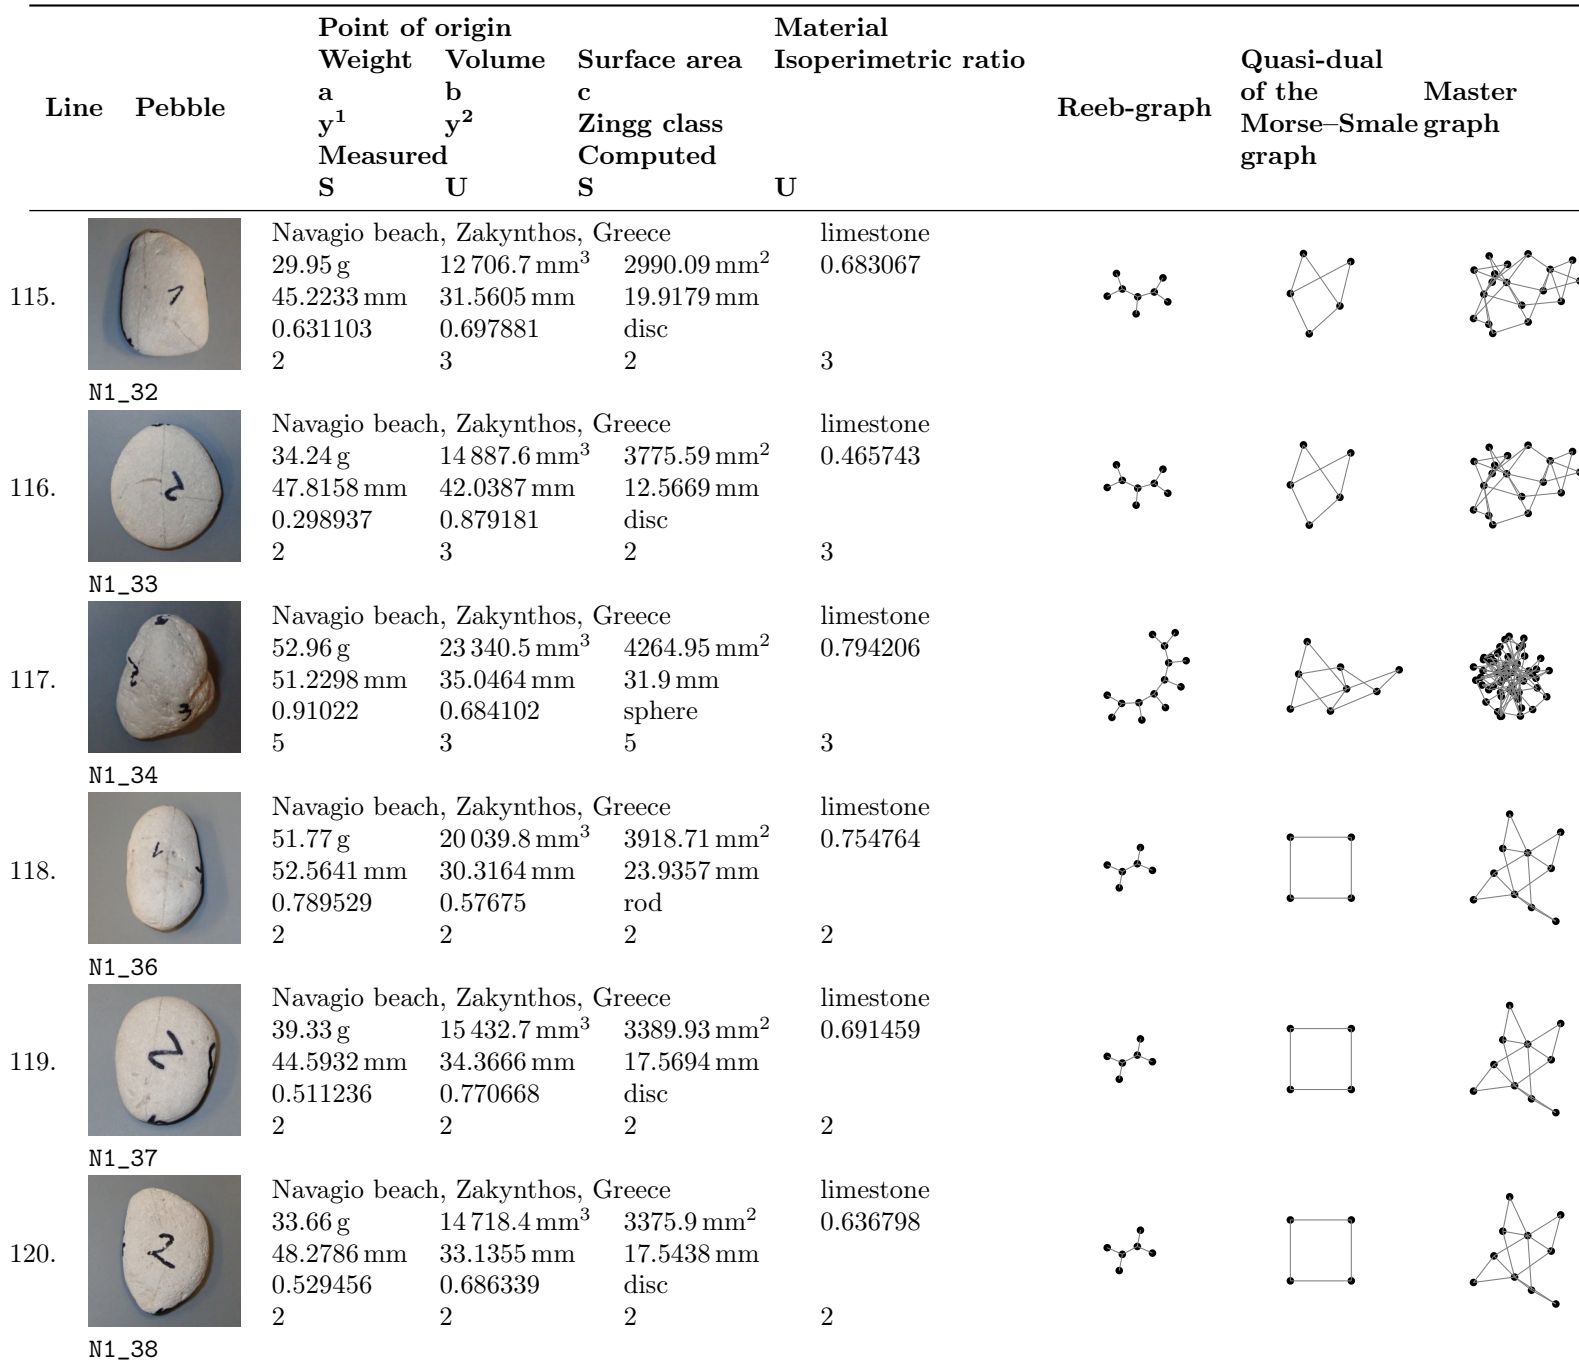 | Navagio beach, Zakynthos, Greece<br>39.33 g<br>44.5932 mm<br>0.511236<br>2 | 15 432.7 mm <sup>3</sup><br>34.3666 mm<br>0.770668<br>2 | 3389.93 mm <sup>2</sup><br>17.5694 mm<br>disc<br>2 | limestone<br>0.691459<br><br>2 | 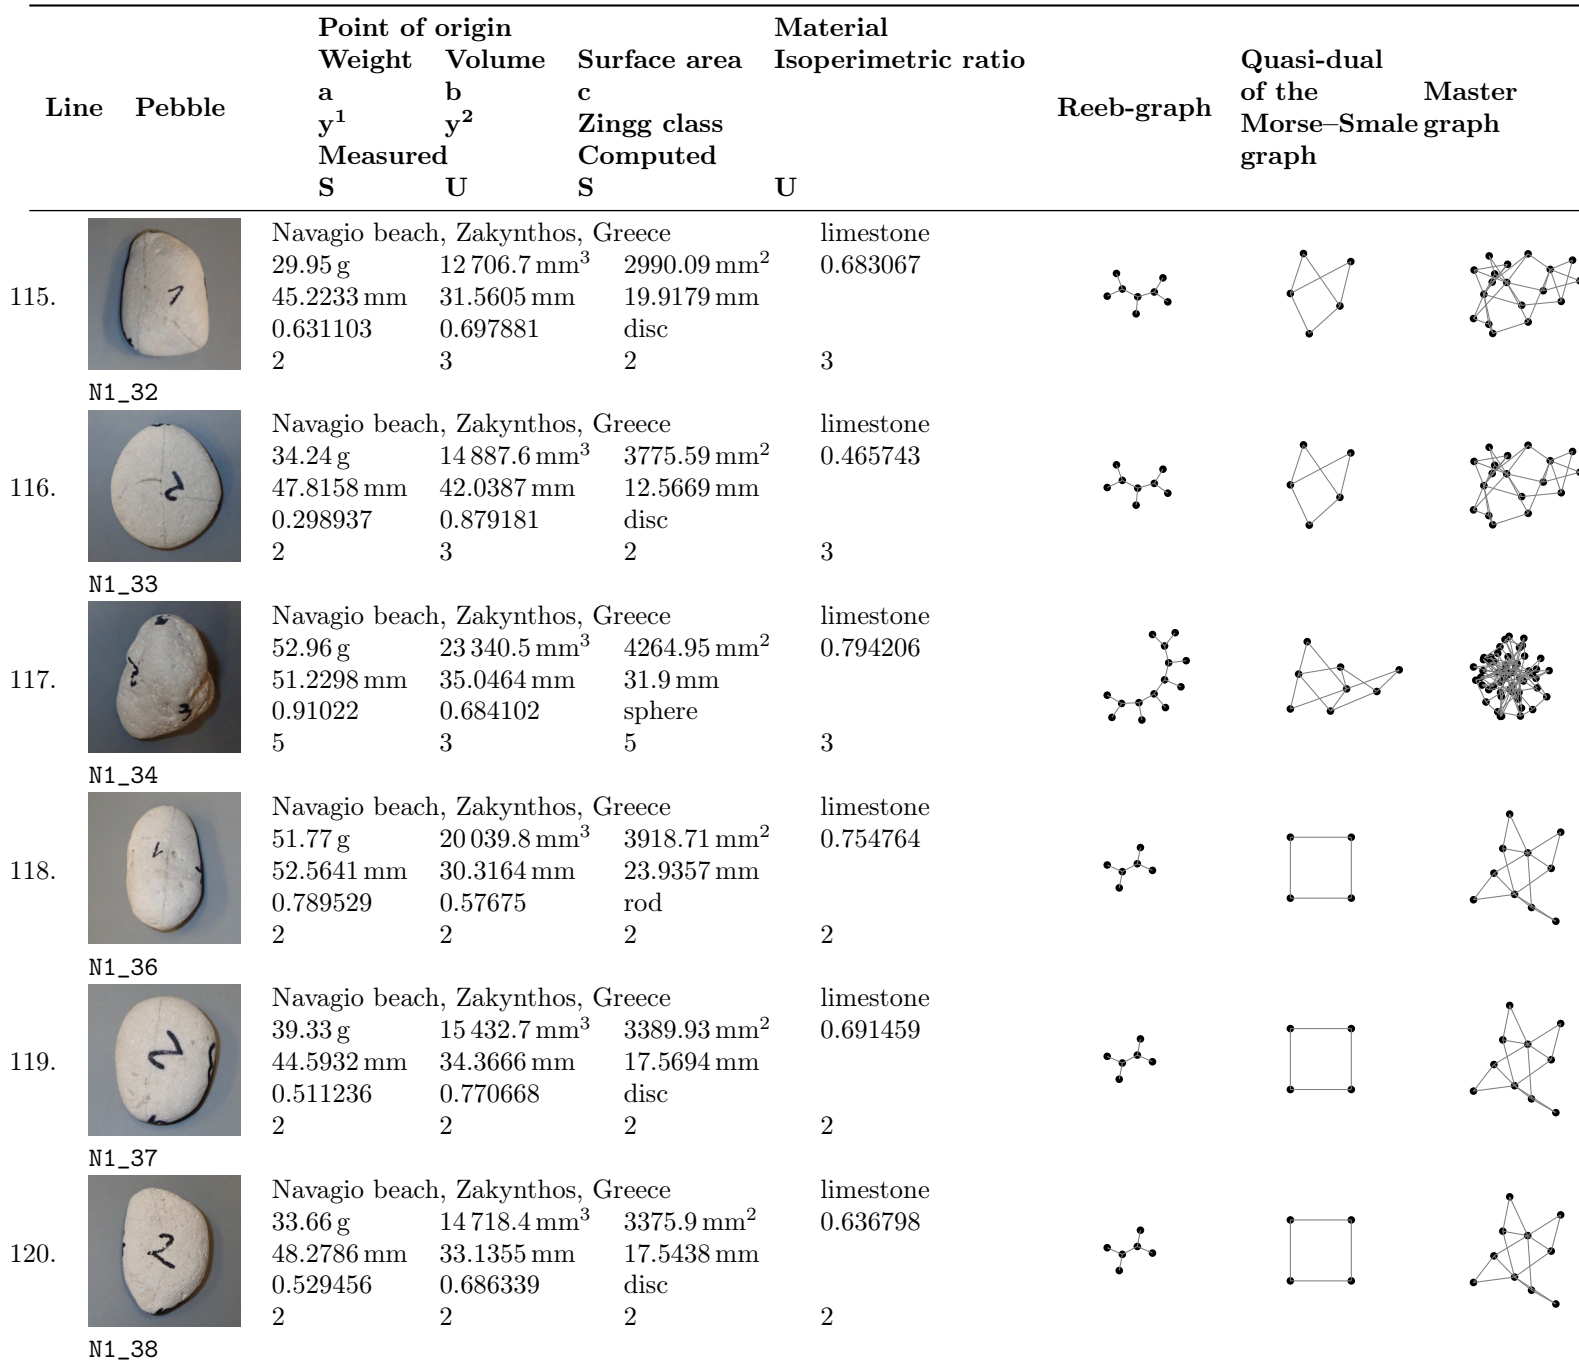 | 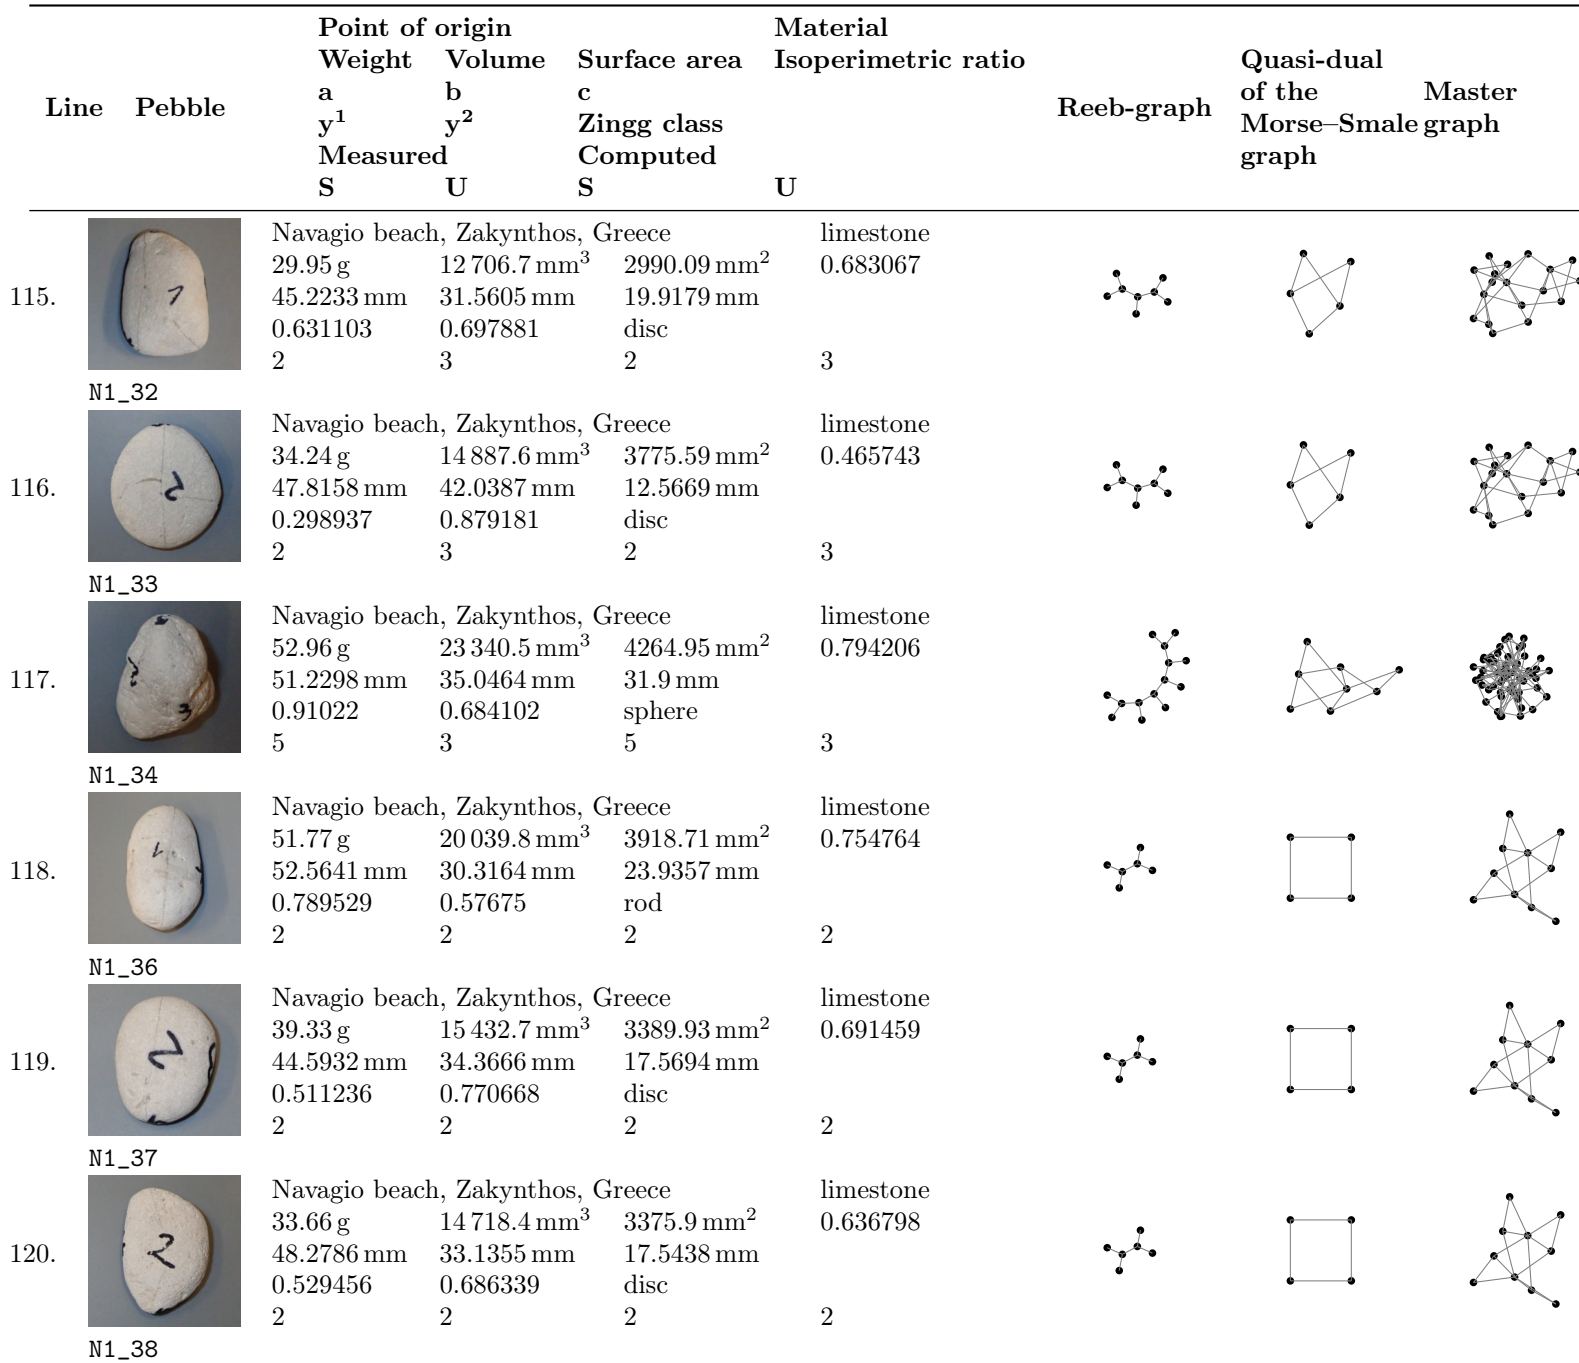 | 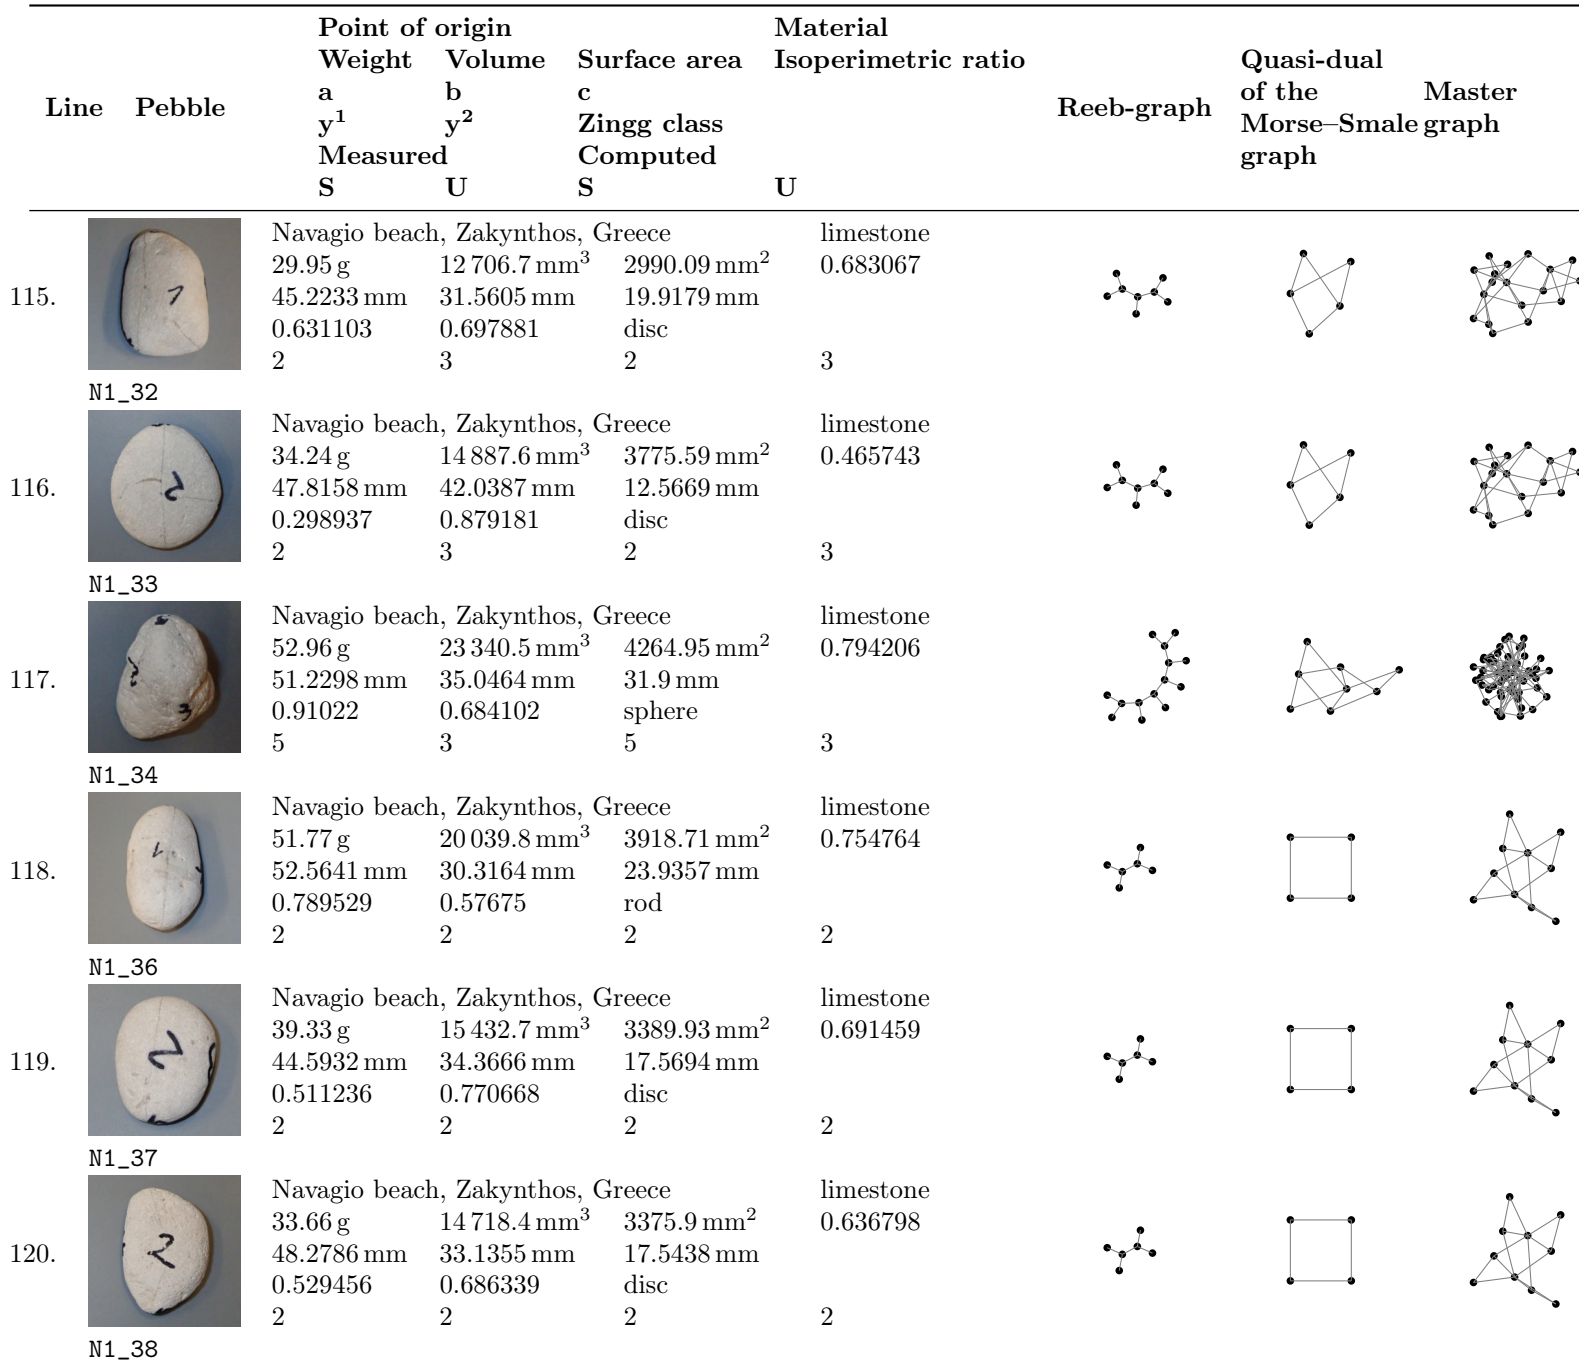 |
|      | N1_37                                                                               |                                                                            |                                                         |                                                    |                                |                                                                                       |                                                                                       |                                                                                       |
| 120. | 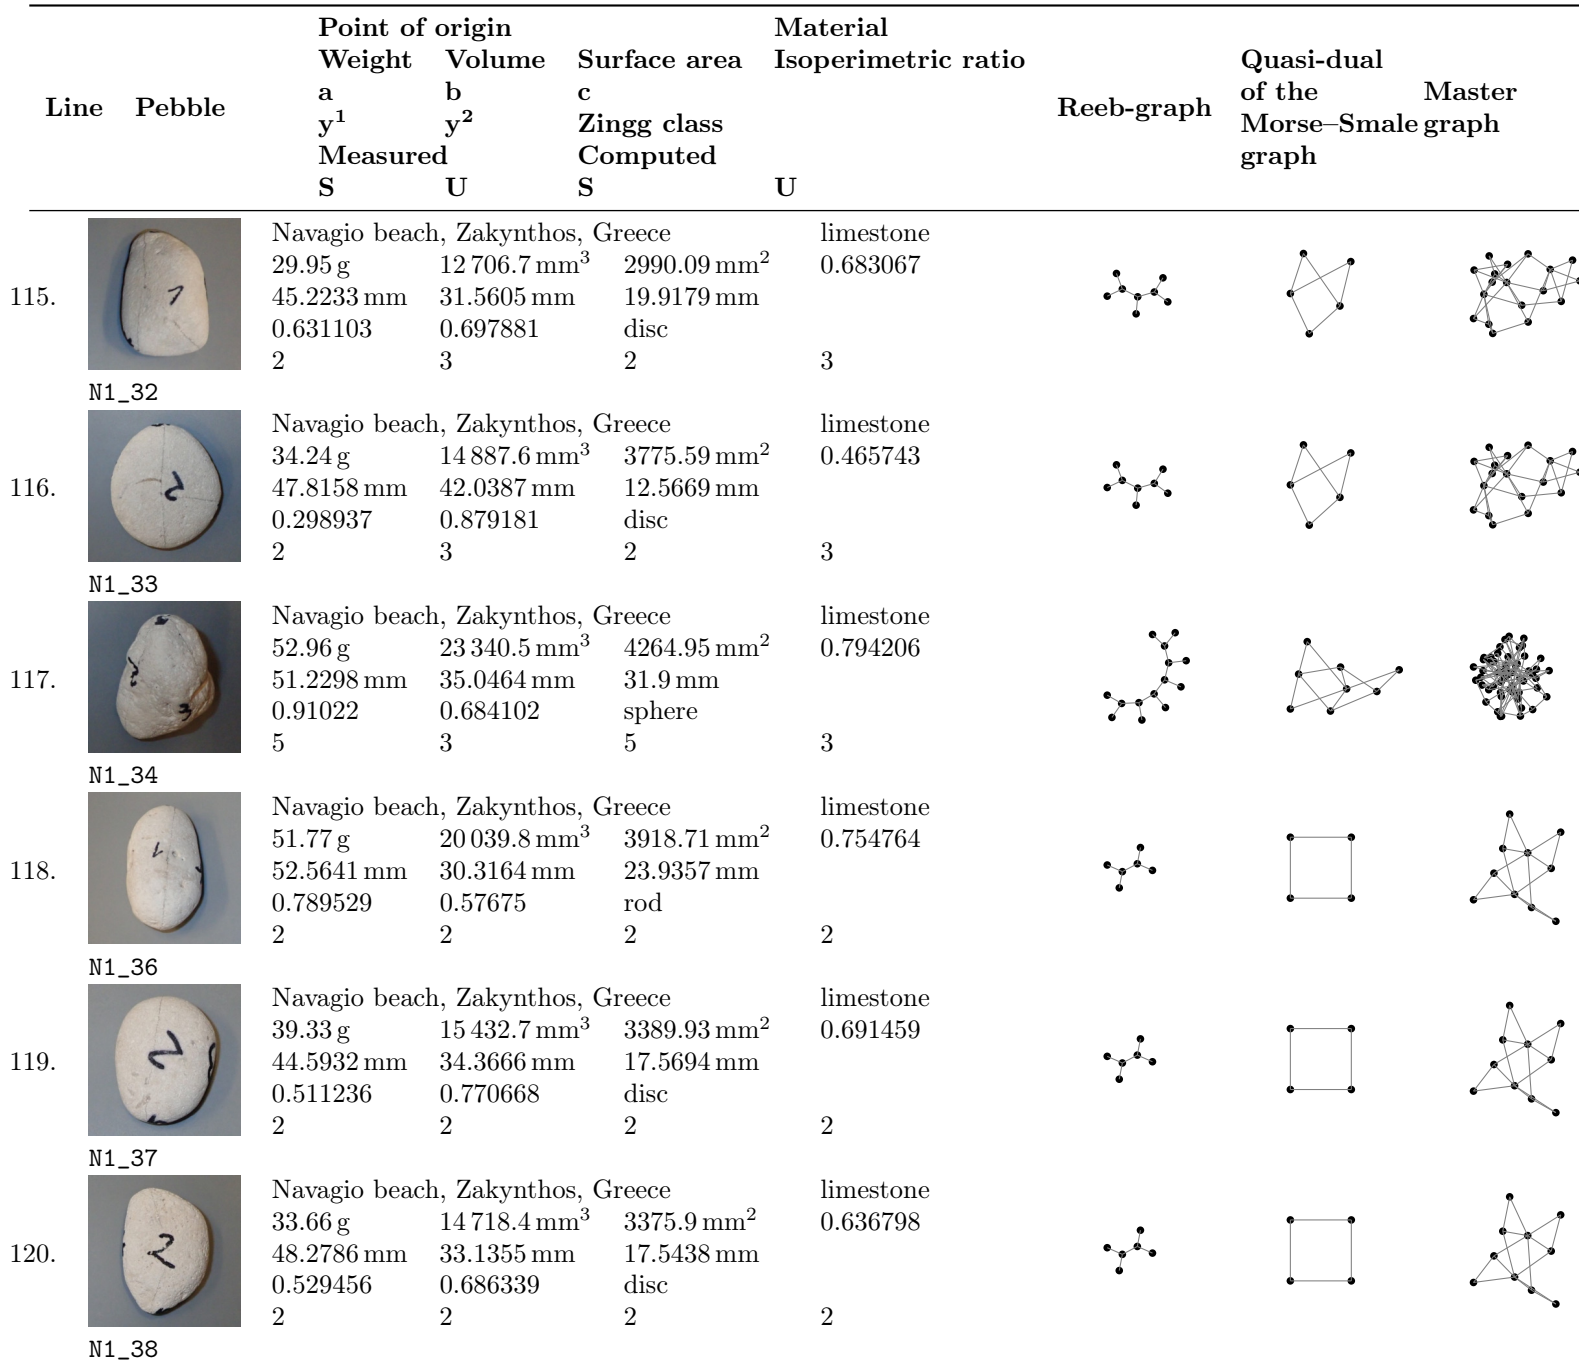 | Navagio beach, Zakynthos, Greece<br>33.66 g<br>48.2786 mm<br>0.529456<br>2 | 14 718.4 mm <sup>3</sup><br>33.1355 mm<br>0.686339<br>2 | 3375.9 mm <sup>2</sup><br>17.5438 mm<br>disc<br>2  | limestone<br>0.636798<br><br>2 | 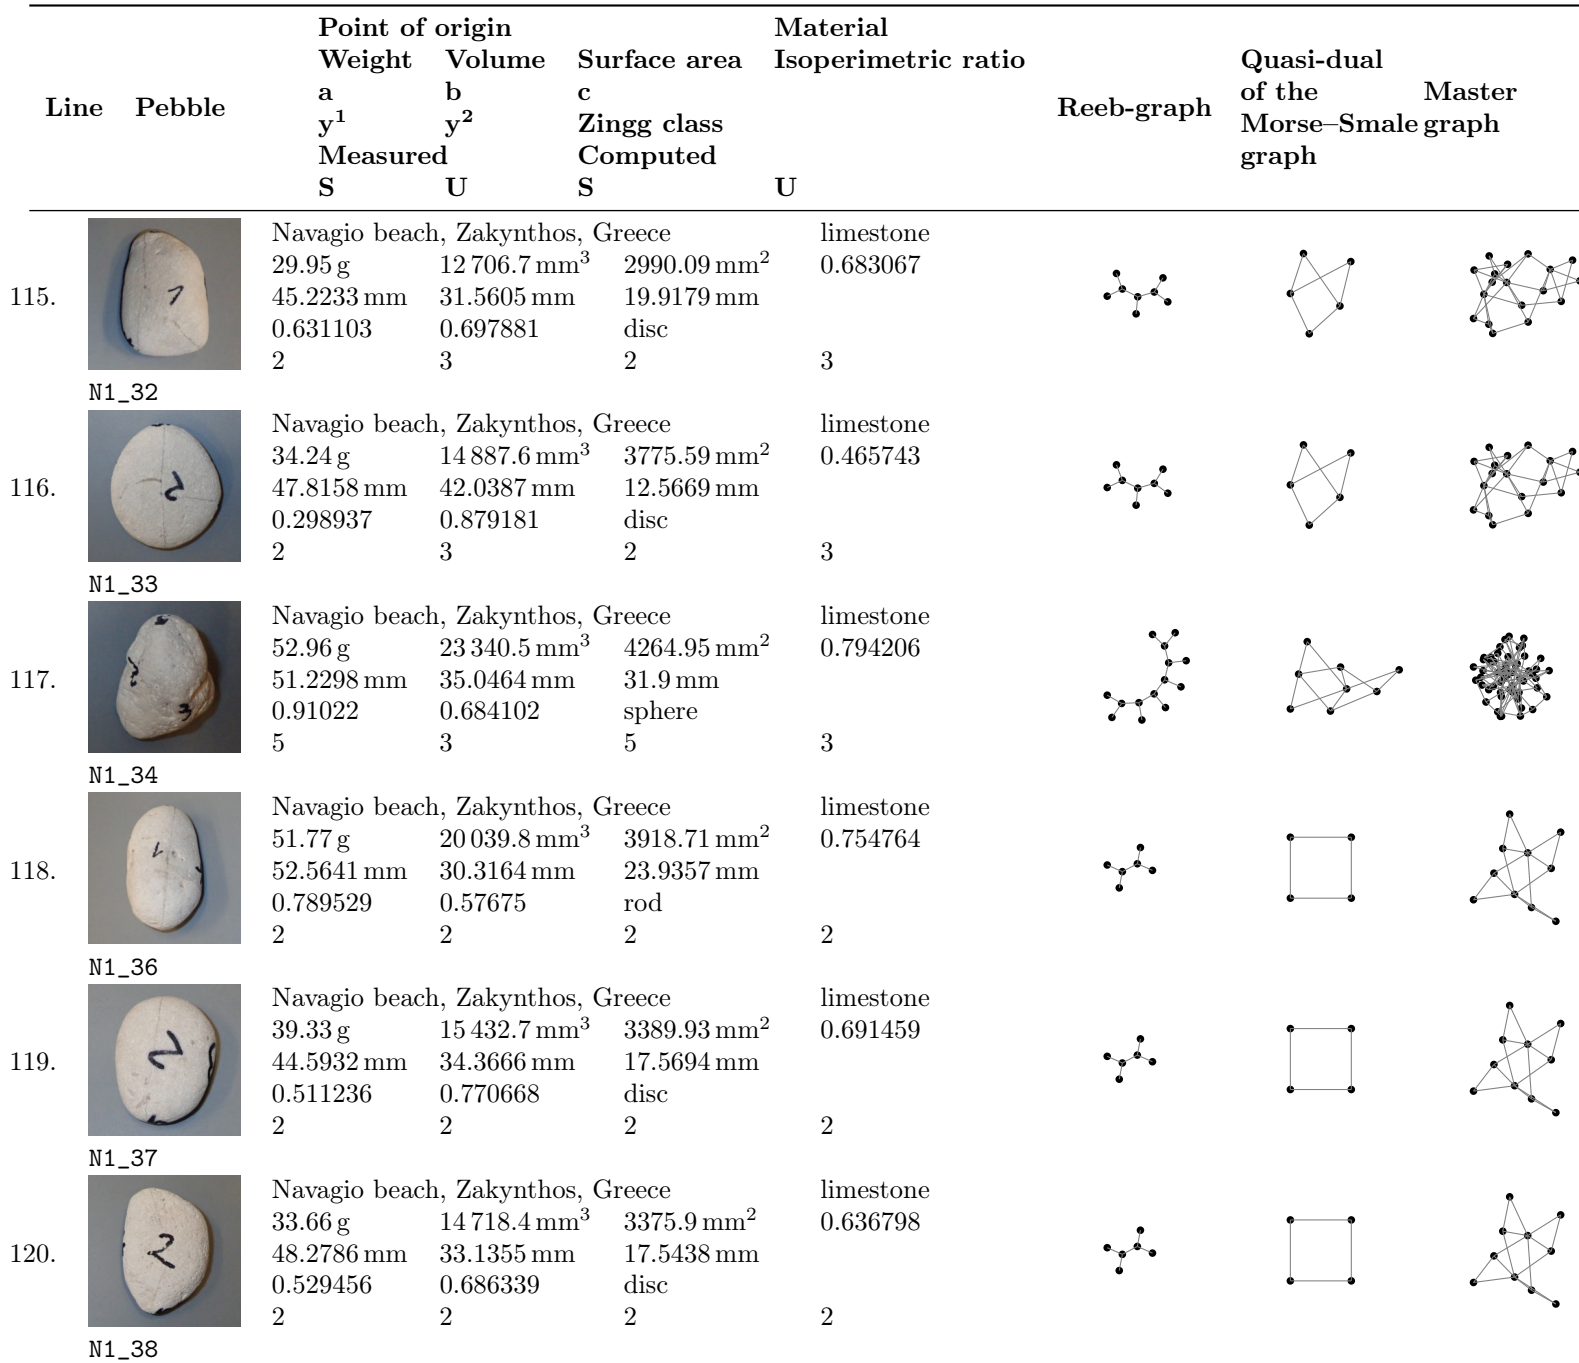 | 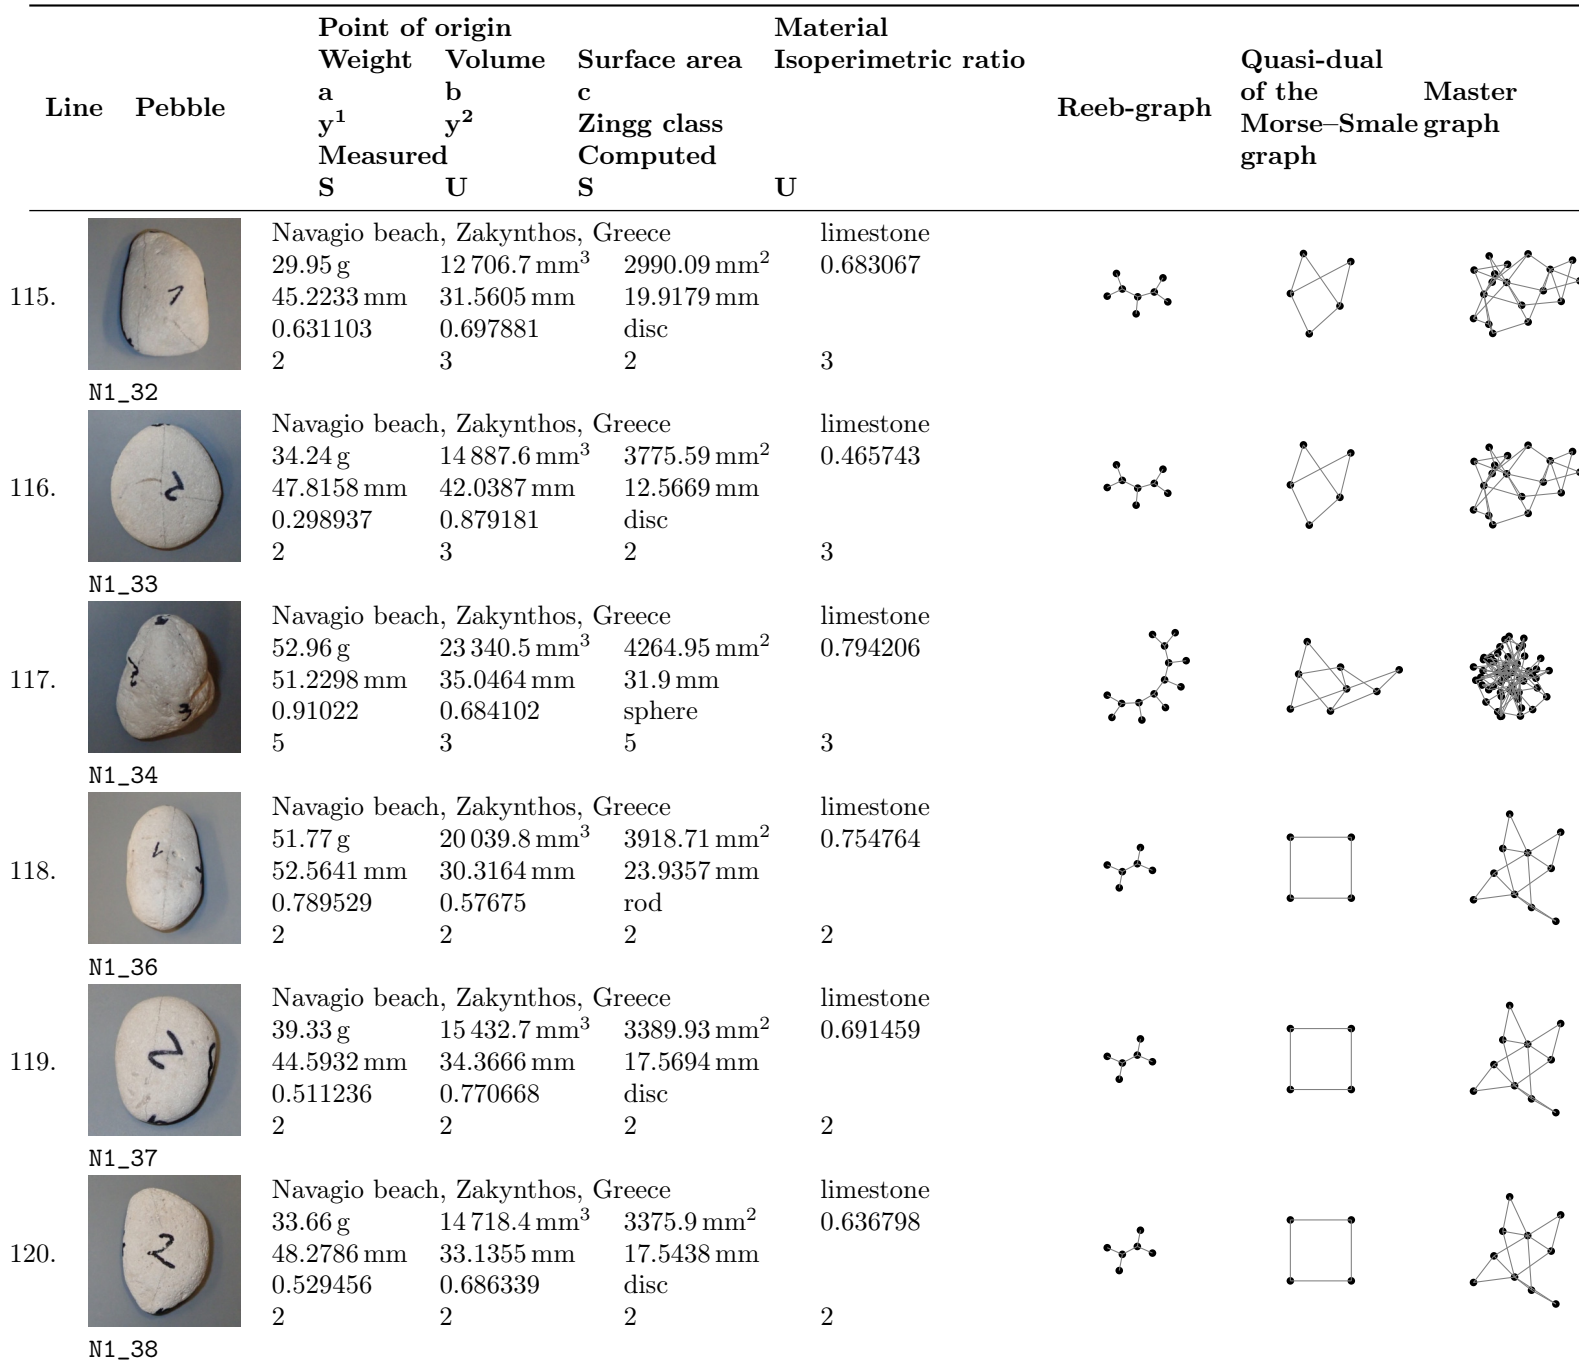 | 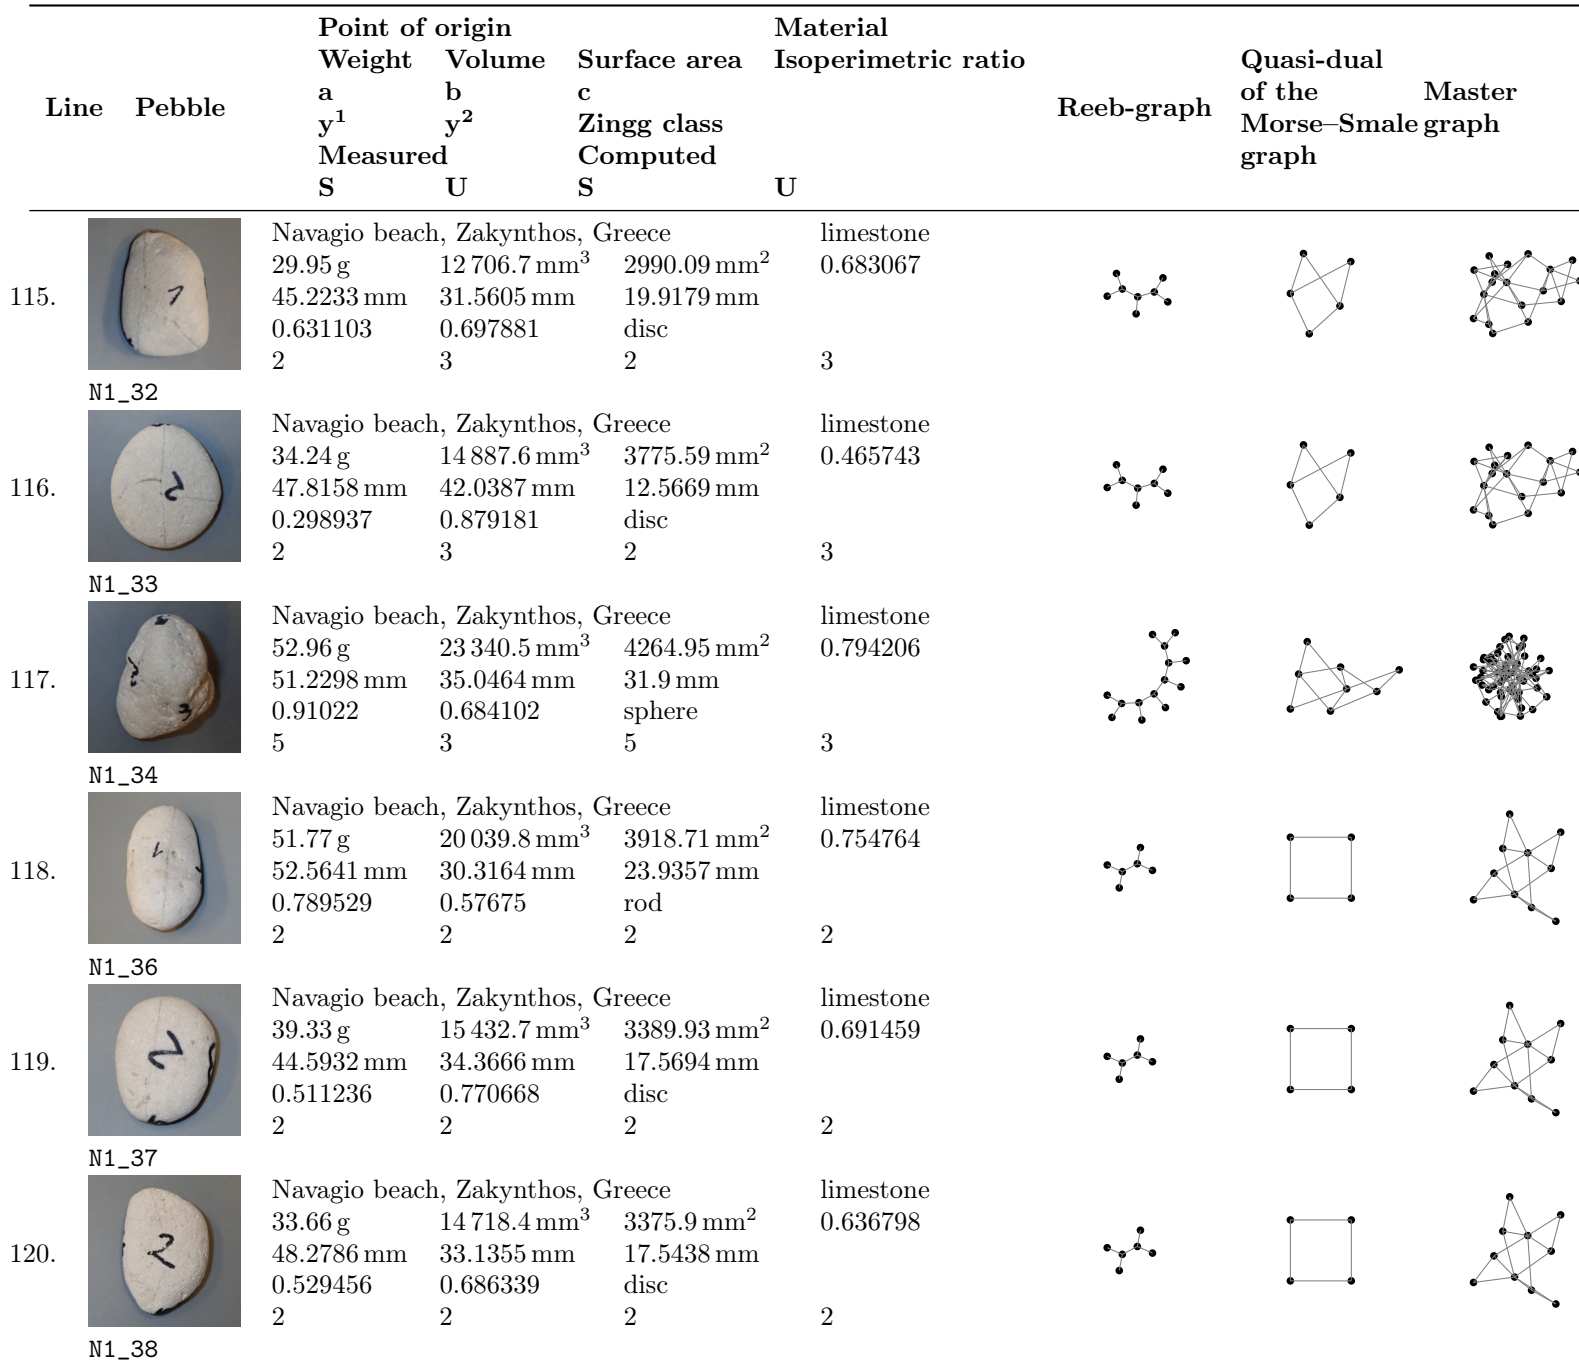 |
|      | N1_38                                                                               |                                                                            |                                                         |                                                    |                                |                                                                                       |                                                                                       |                                                                                       |

| Line | Pebble                                                                              | Point of origin                                                            |                                                         |                                                     | Material                       | Reeb-graph                                                                            | Quasi-dual<br>of the<br>Morse–Smale<br>graph                                          | Master                                                                                |
|------|-------------------------------------------------------------------------------------|----------------------------------------------------------------------------|---------------------------------------------------------|-----------------------------------------------------|--------------------------------|---------------------------------------------------------------------------------------|---------------------------------------------------------------------------------------|---------------------------------------------------------------------------------------|
|      |                                                                                     | Weight                                                                     | Volume                                                  | Surface area                                        |                                |                                                                                       |                                                                                       |                                                                                       |
|      |                                                                                     | a                                                                          | b                                                       | c                                                   |                                |                                                                                       |                                                                                       |                                                                                       |
|      |                                                                                     | y <sup>1</sup><br>Measured<br>S                                            | y <sup>2</sup><br>U                                     | Zingg class<br>Computed<br>S                        |                                |                                                                                       |                                                                                       |                                                                                       |
| 121. | 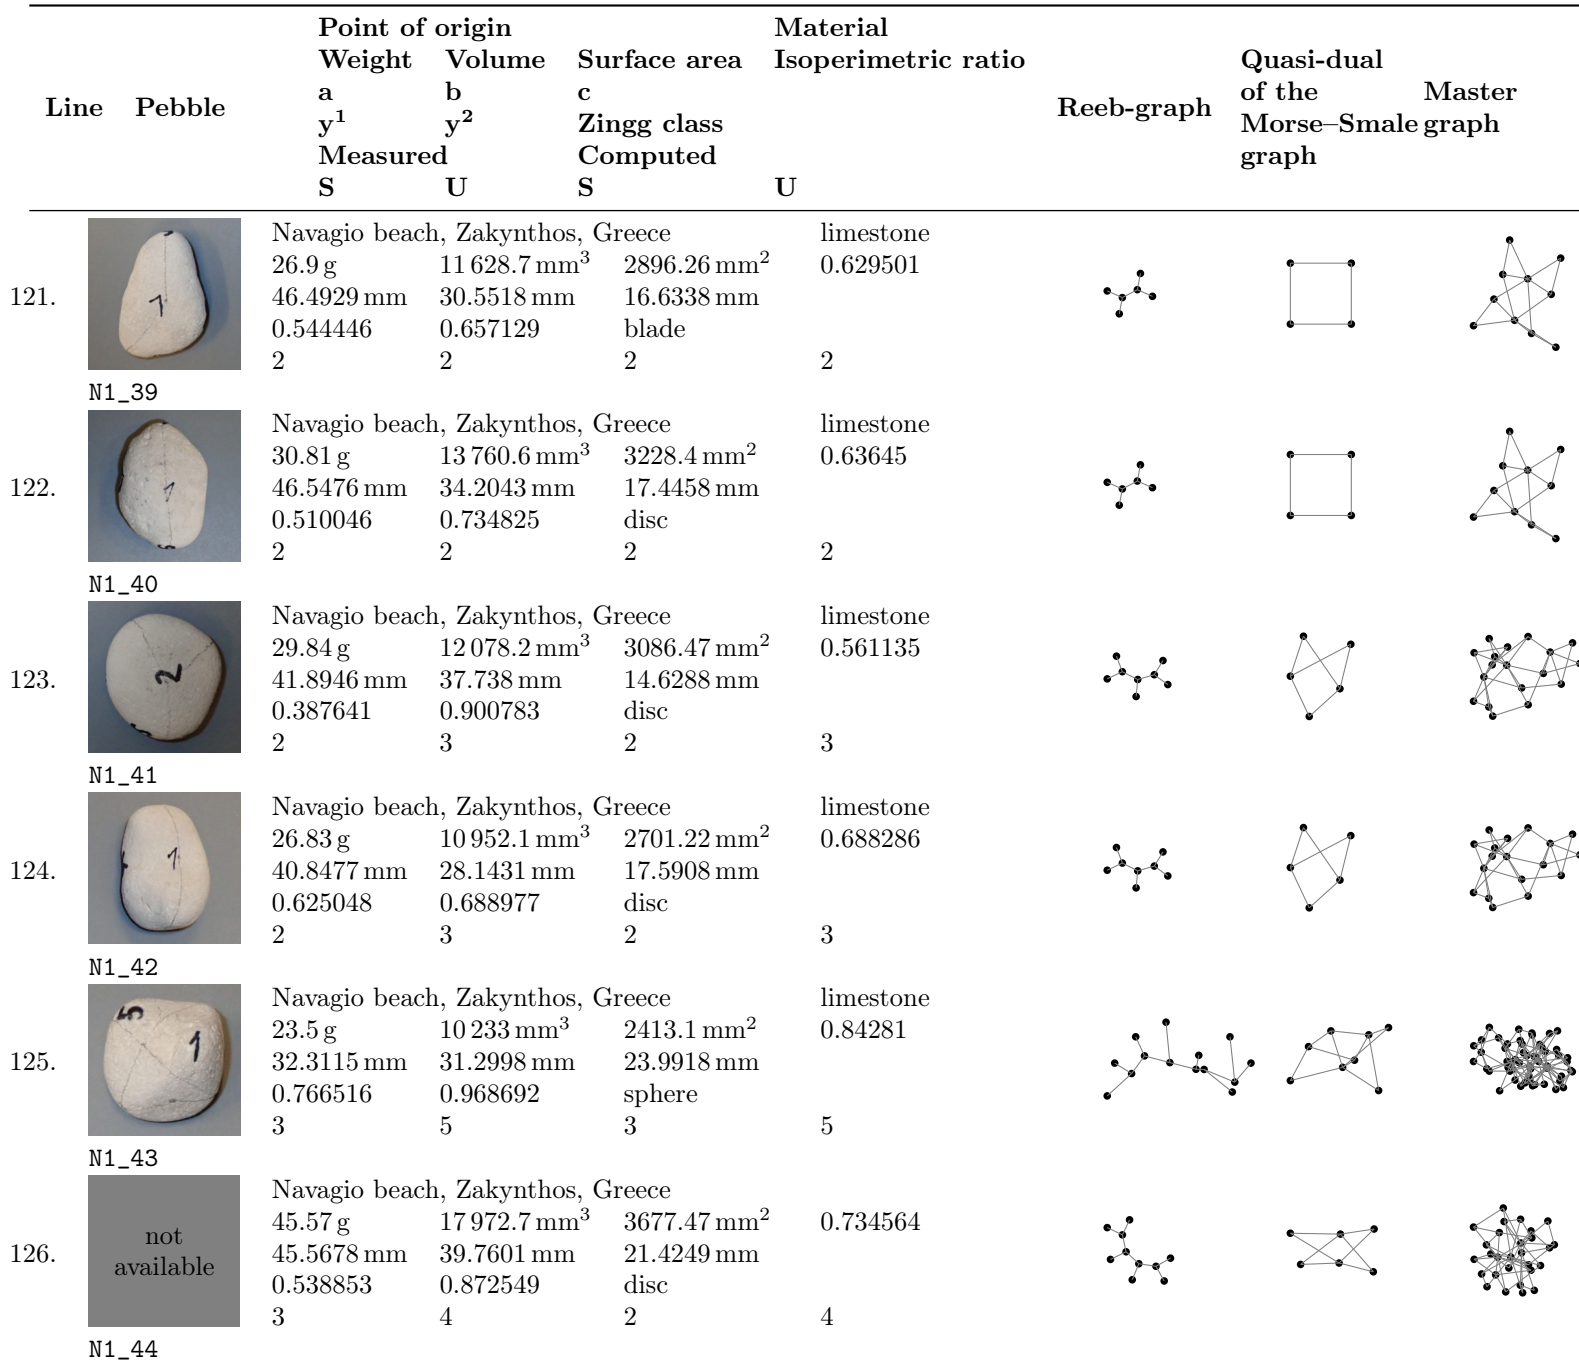   | Navagio beach, Zakynthos, Greece<br>26.9 g<br>46.4929 mm<br>0.544446<br>2  | 11 628.7 mm <sup>3</sup><br>30.5518 mm<br>0.657129<br>2 | 2896.26 mm <sup>2</sup><br>16.6338 mm<br>blade<br>2 | limestone<br>0.629501<br><br>2 | 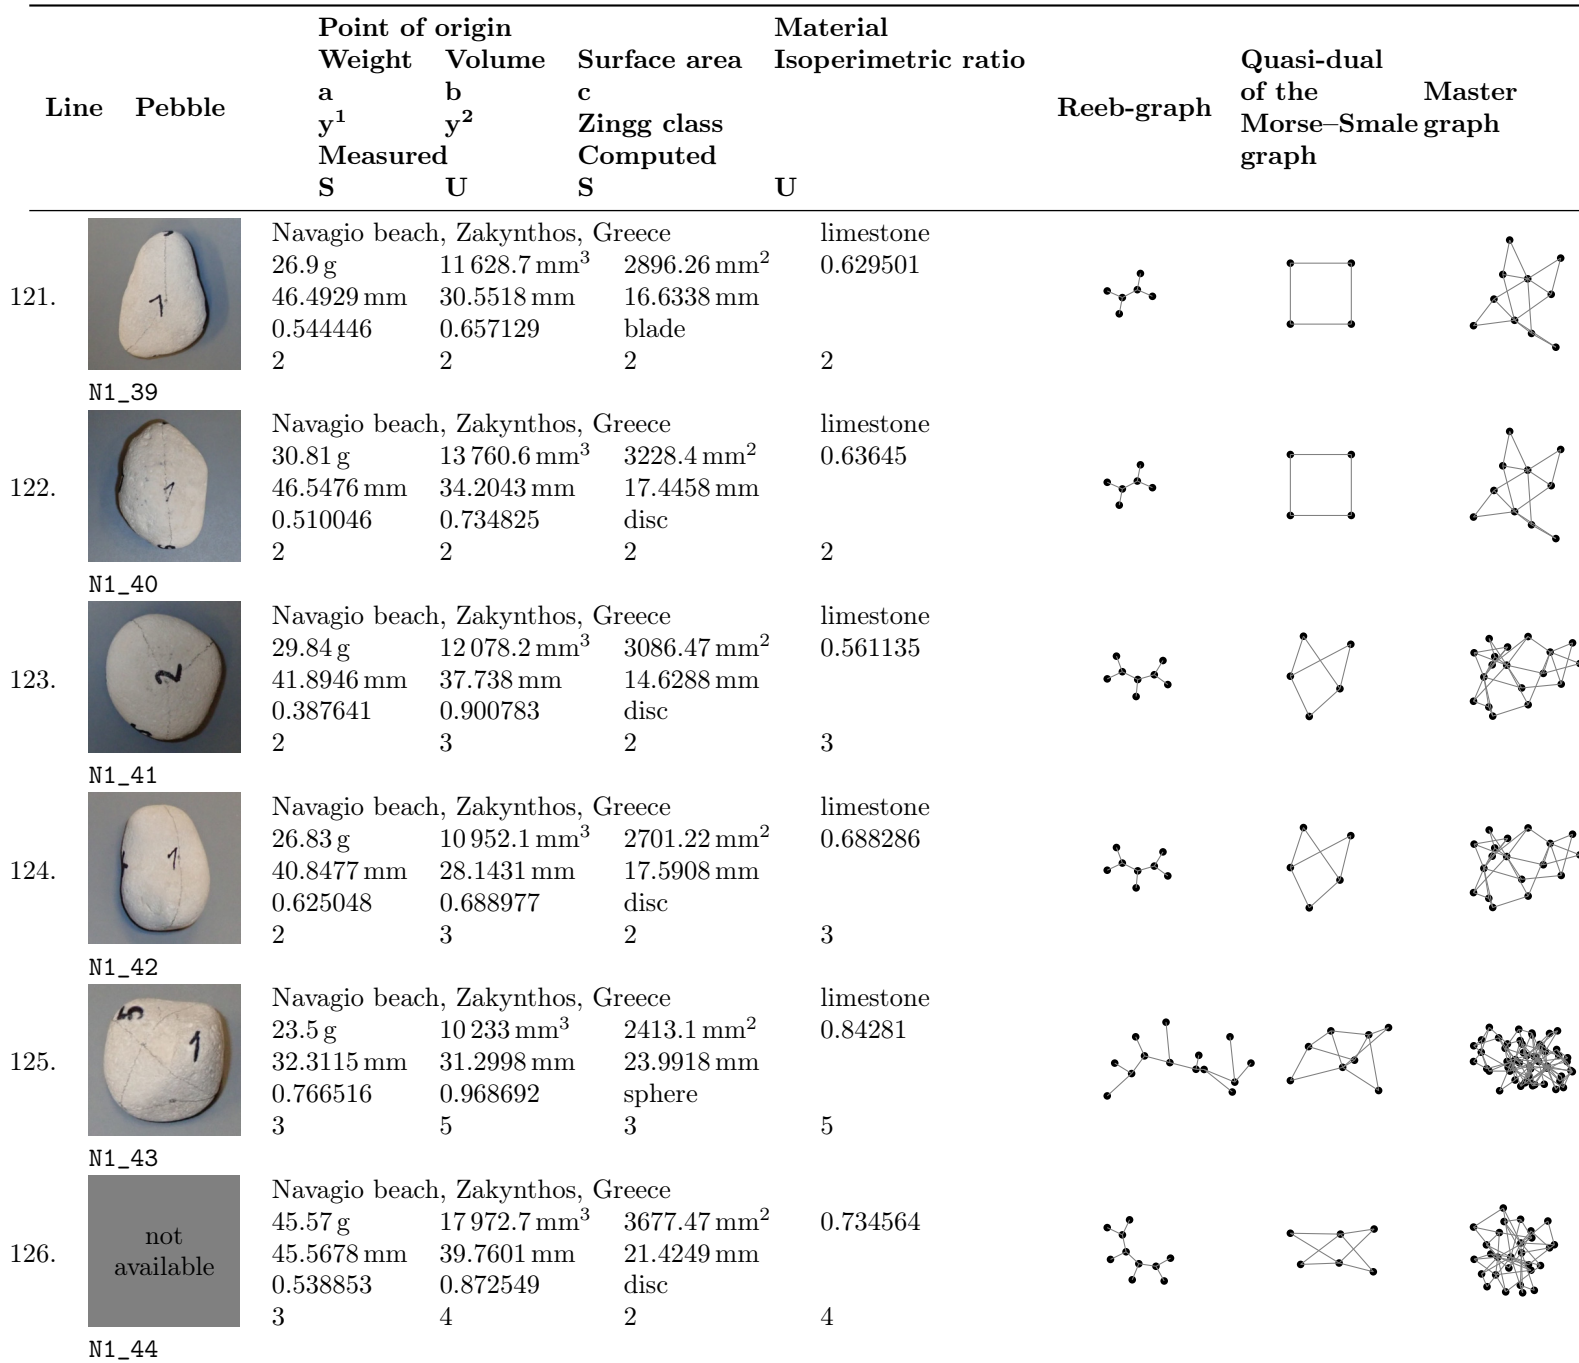   | 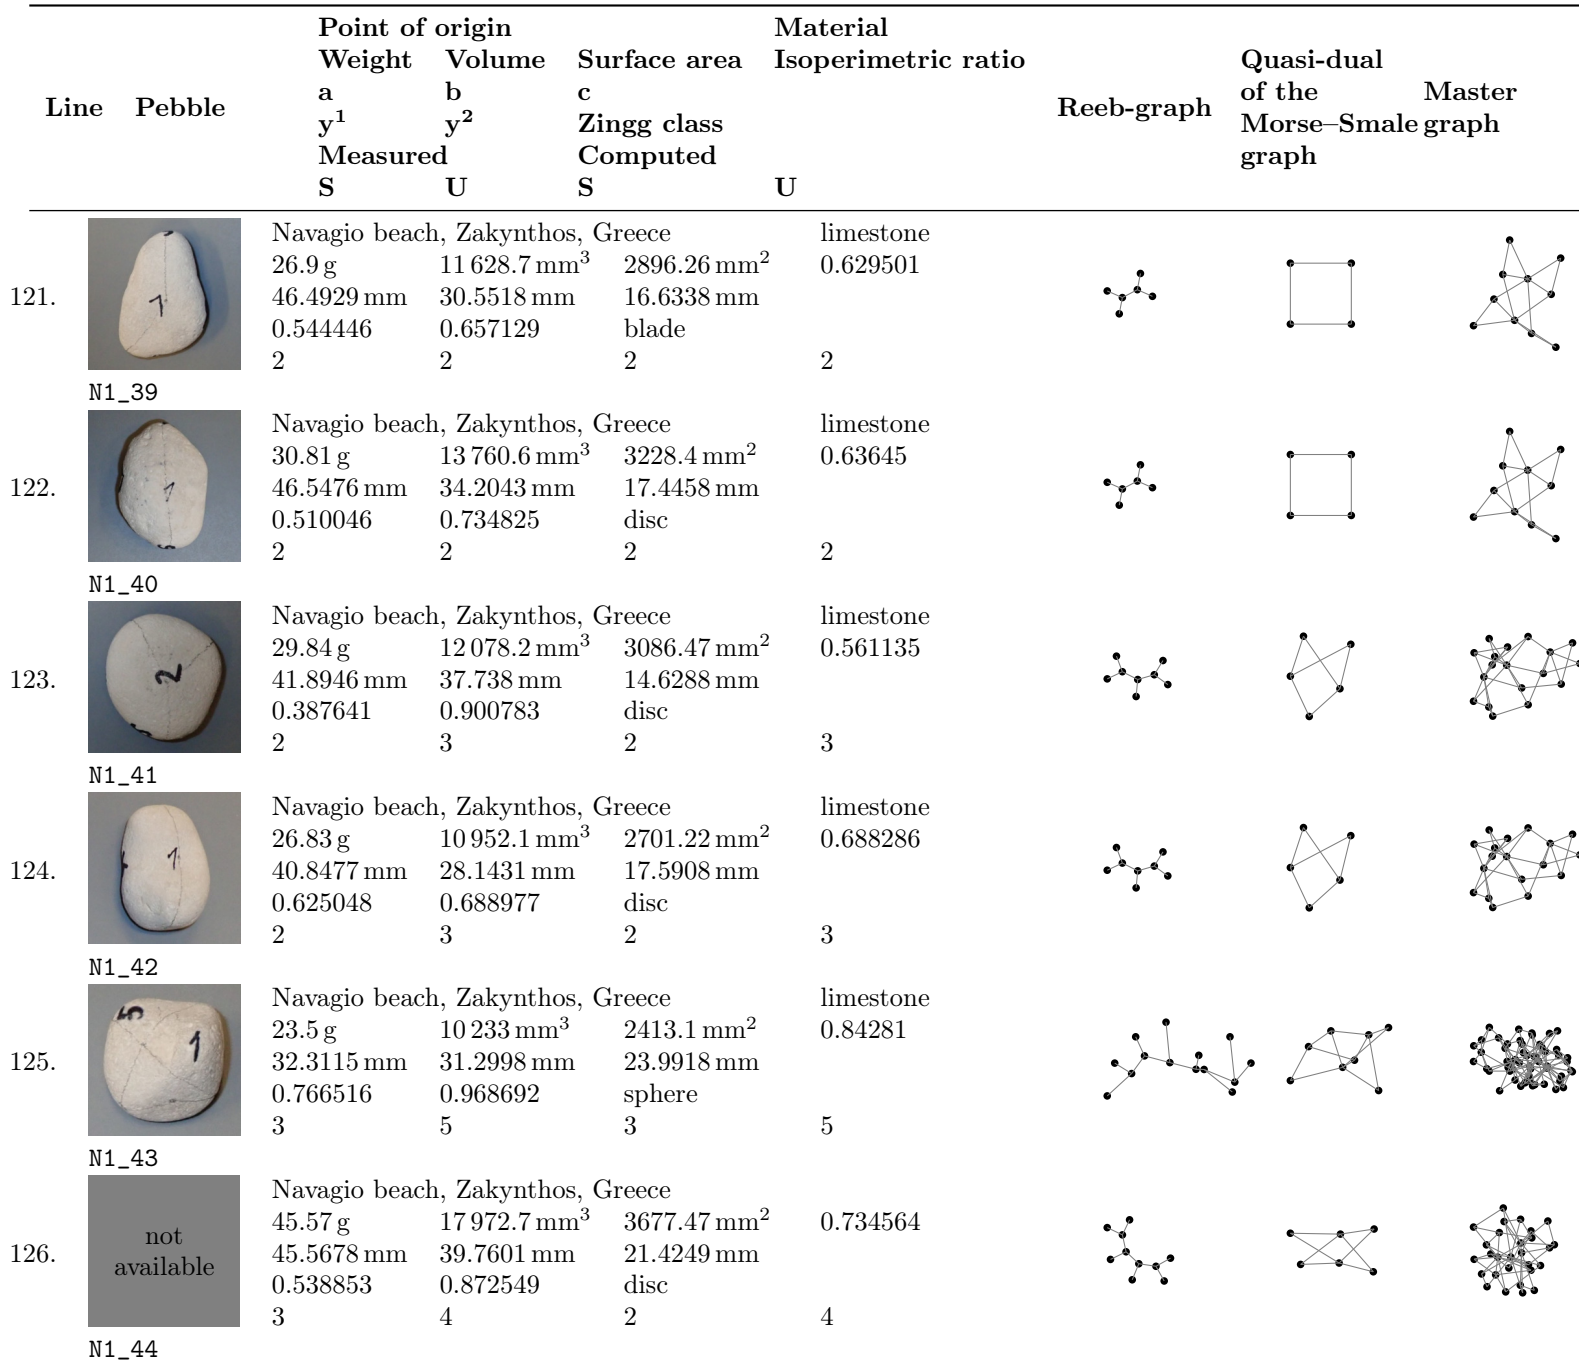   | 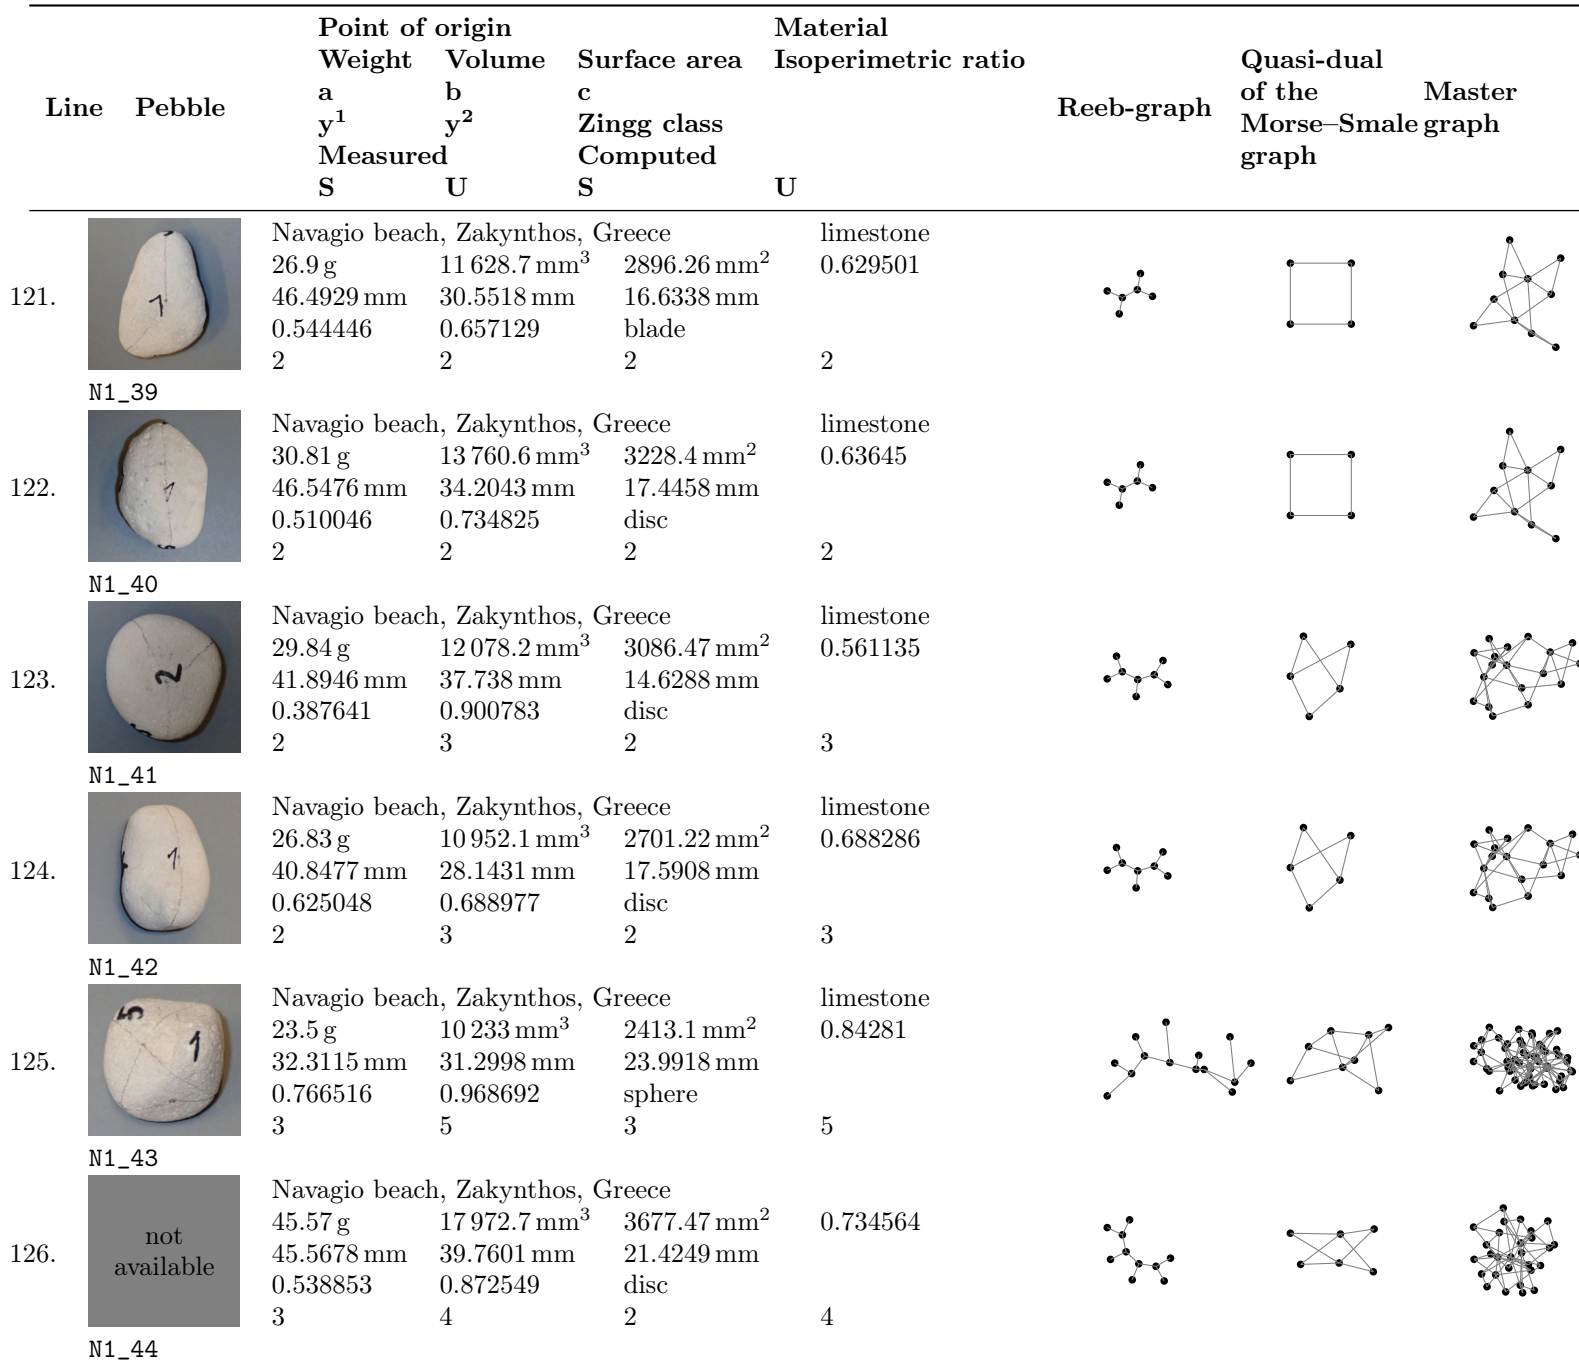   |
|      | N1_39                                                                               |                                                                            |                                                         |                                                     |                                |                                                                                       |                                                                                       |                                                                                       |
| 122. | 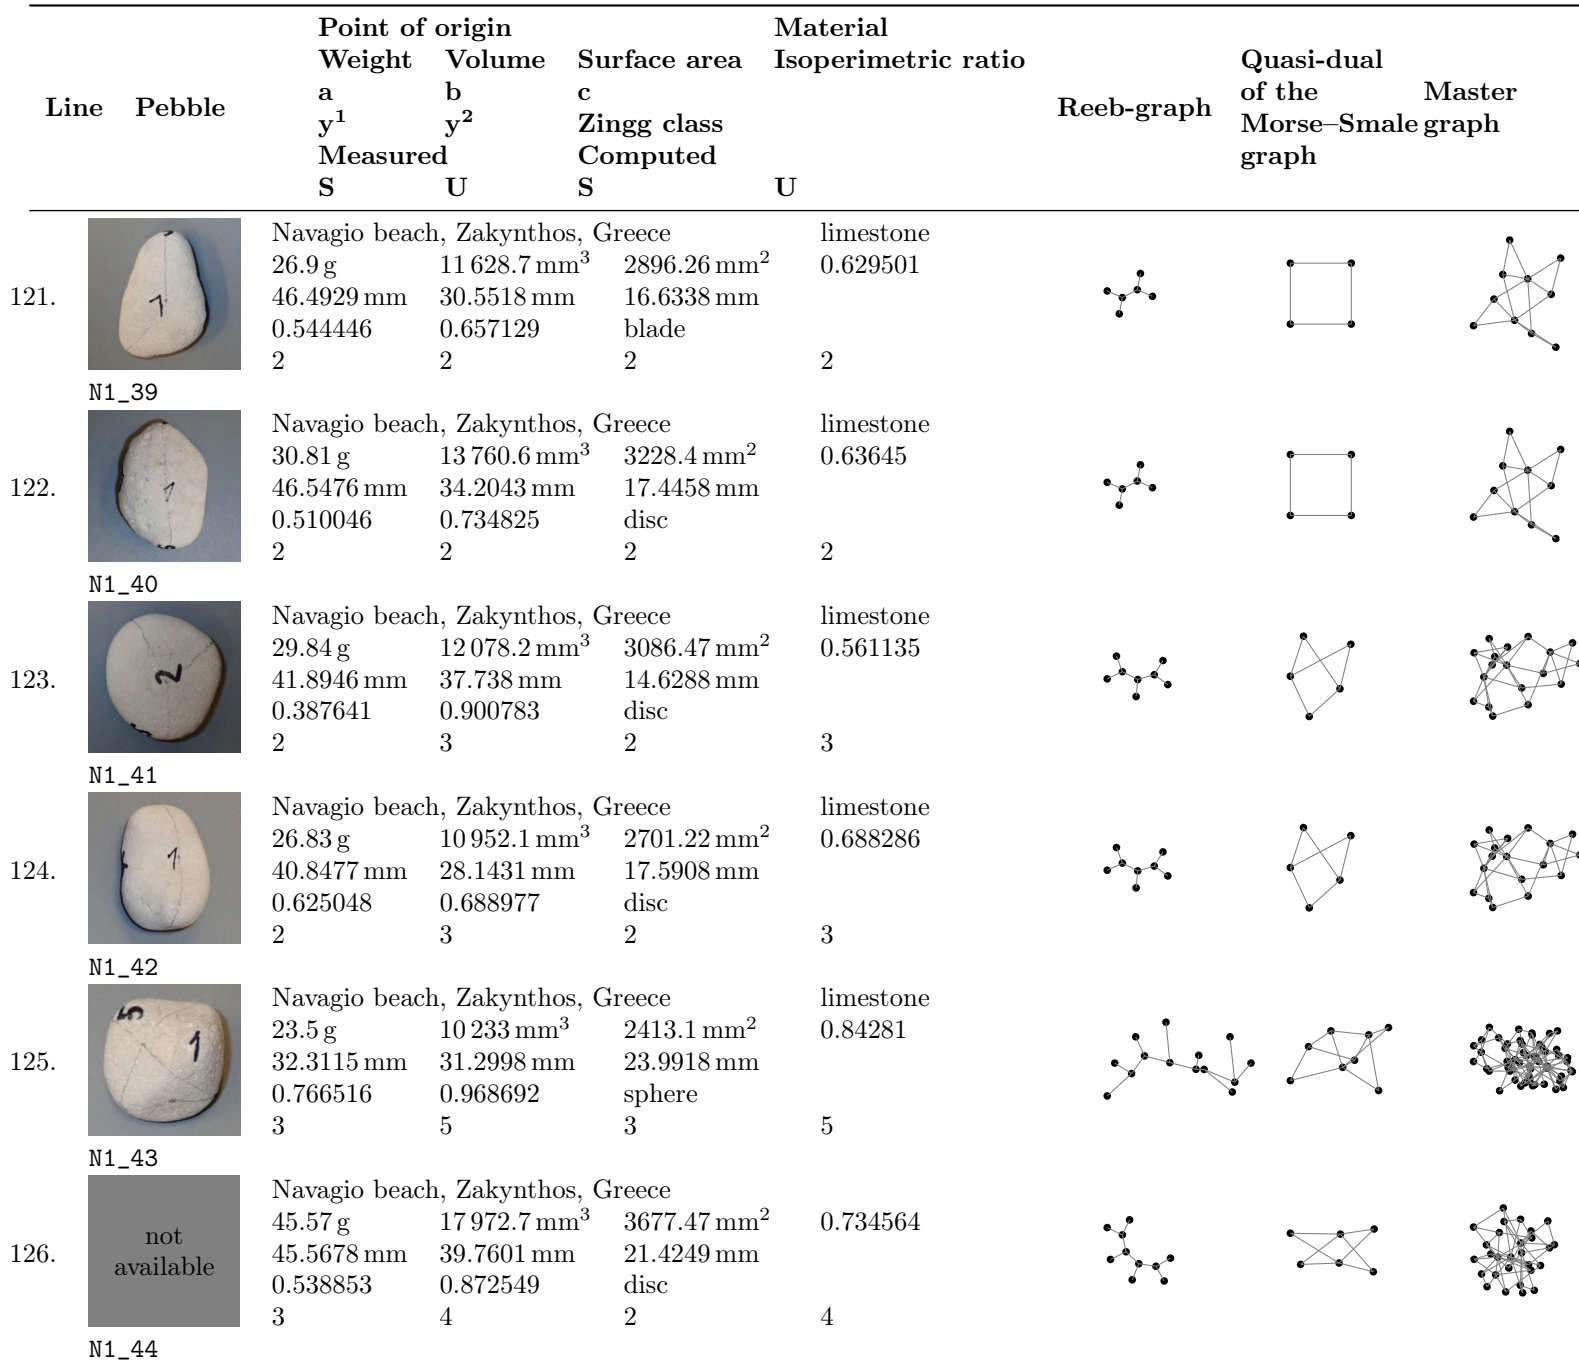   | Navagio beach, Zakynthos, Greece<br>30.81 g<br>46.5476 mm<br>0.510046<br>2 | 13 760.6 mm <sup>3</sup><br>34.2043 mm<br>0.734825<br>2 | 3228.4 mm <sup>2</sup><br>17.4458 mm<br>disc<br>2   | limestone<br>0.63645<br><br>2  | 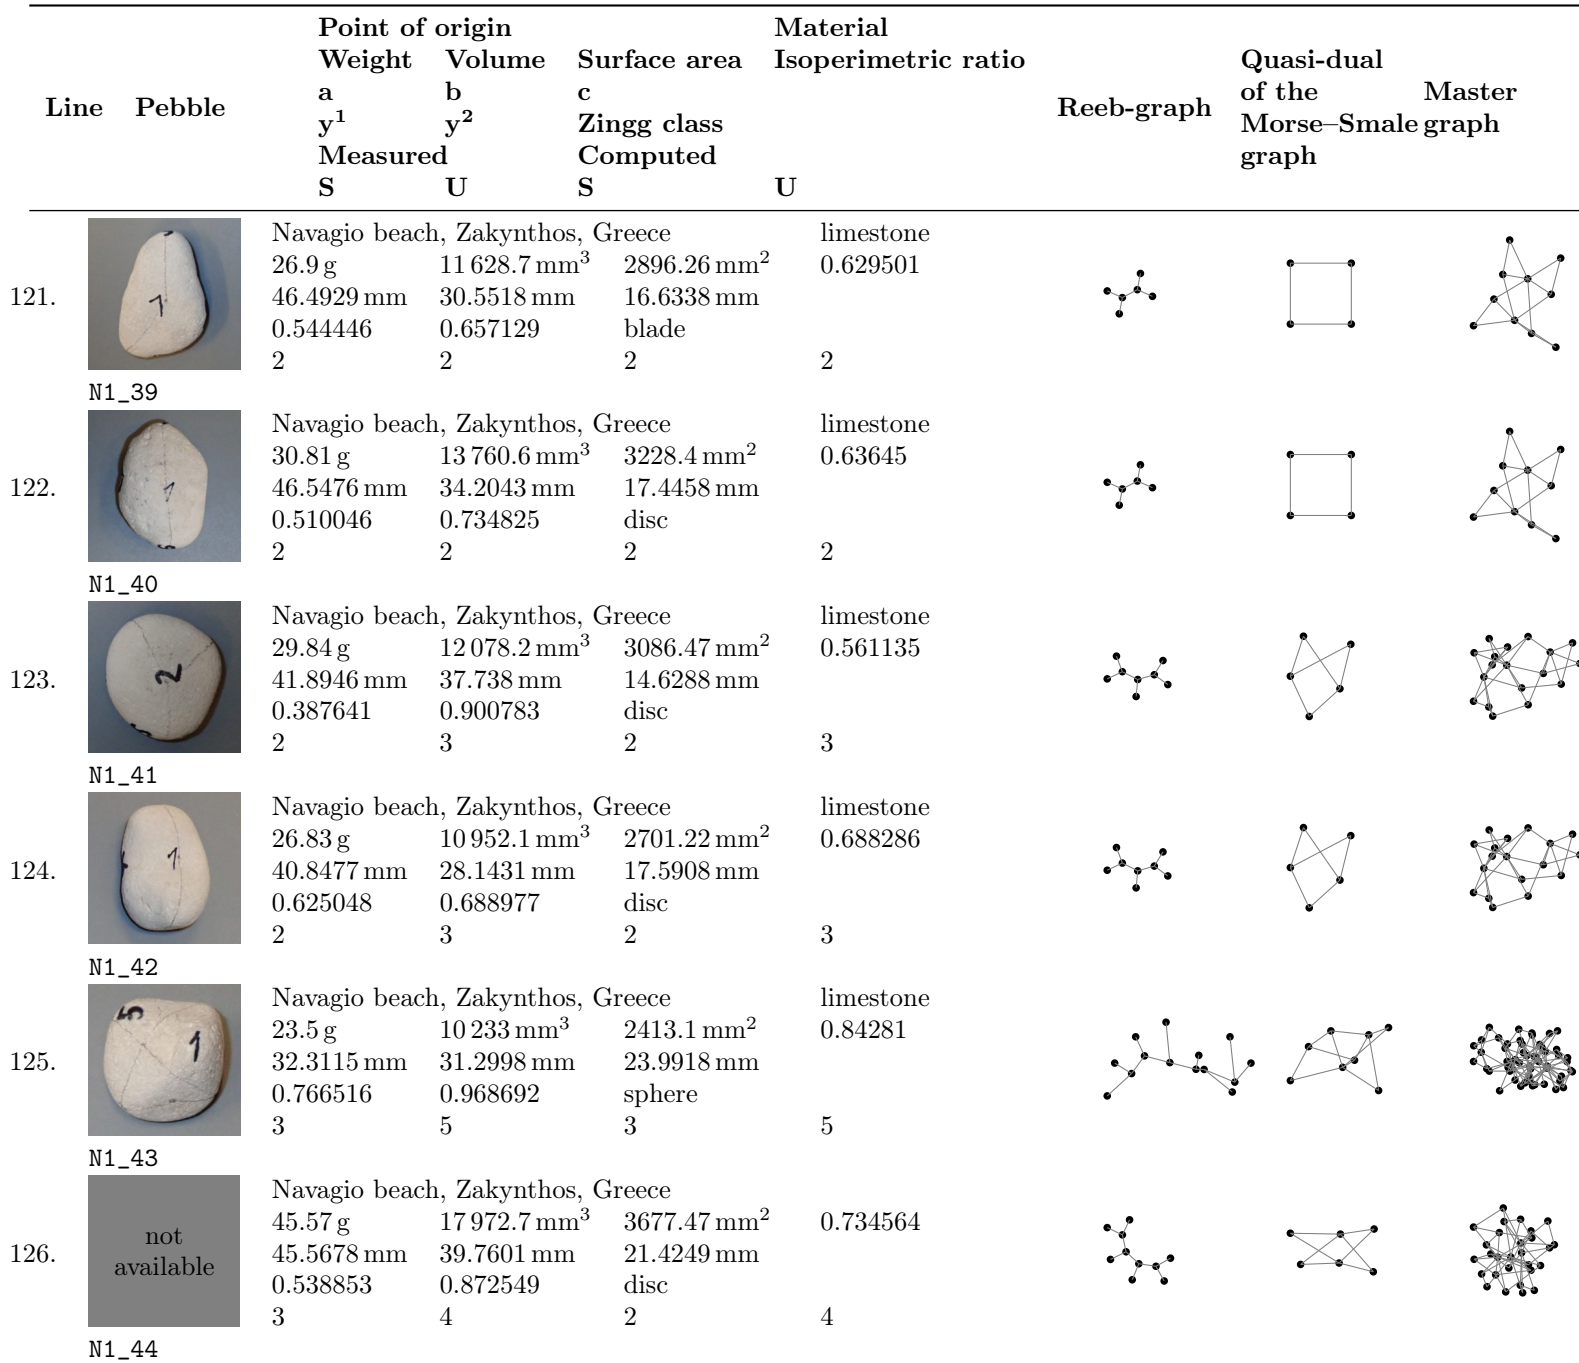   | 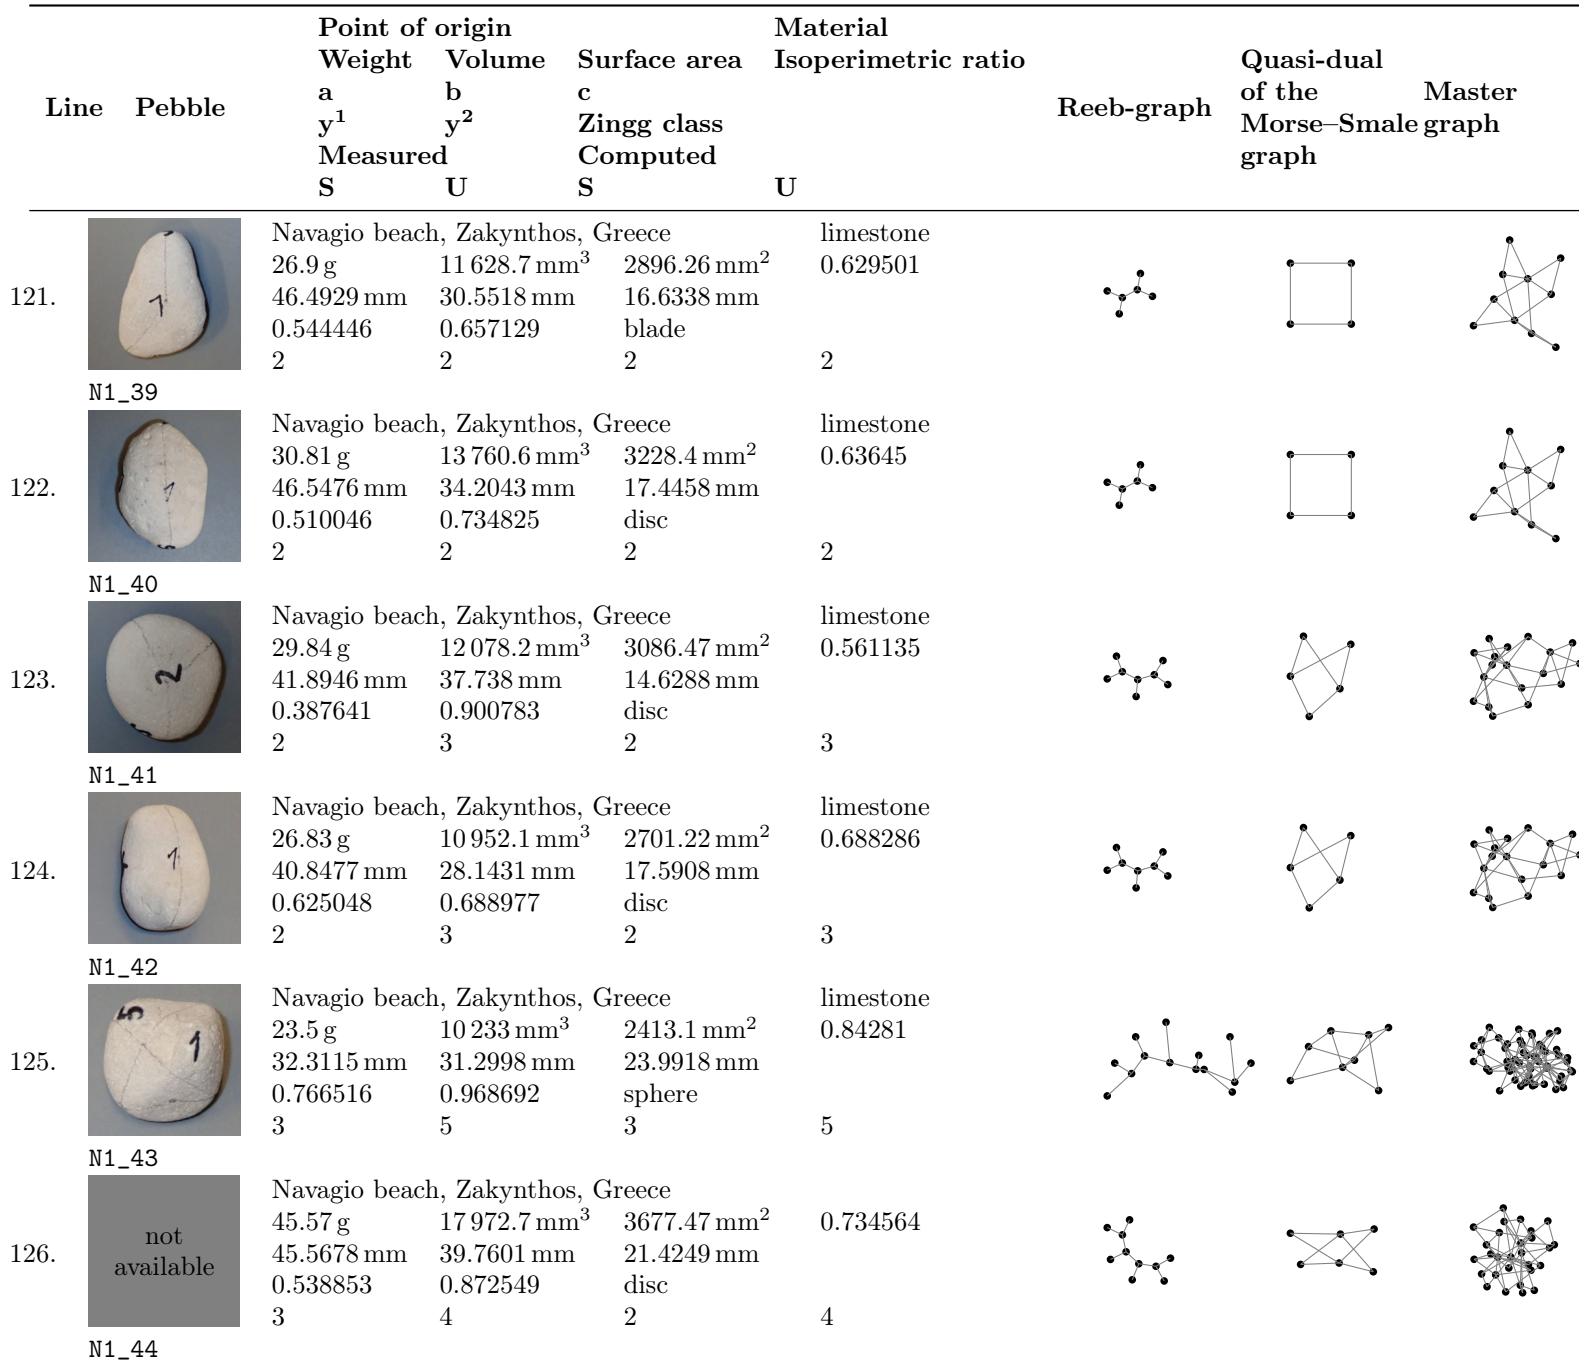   | 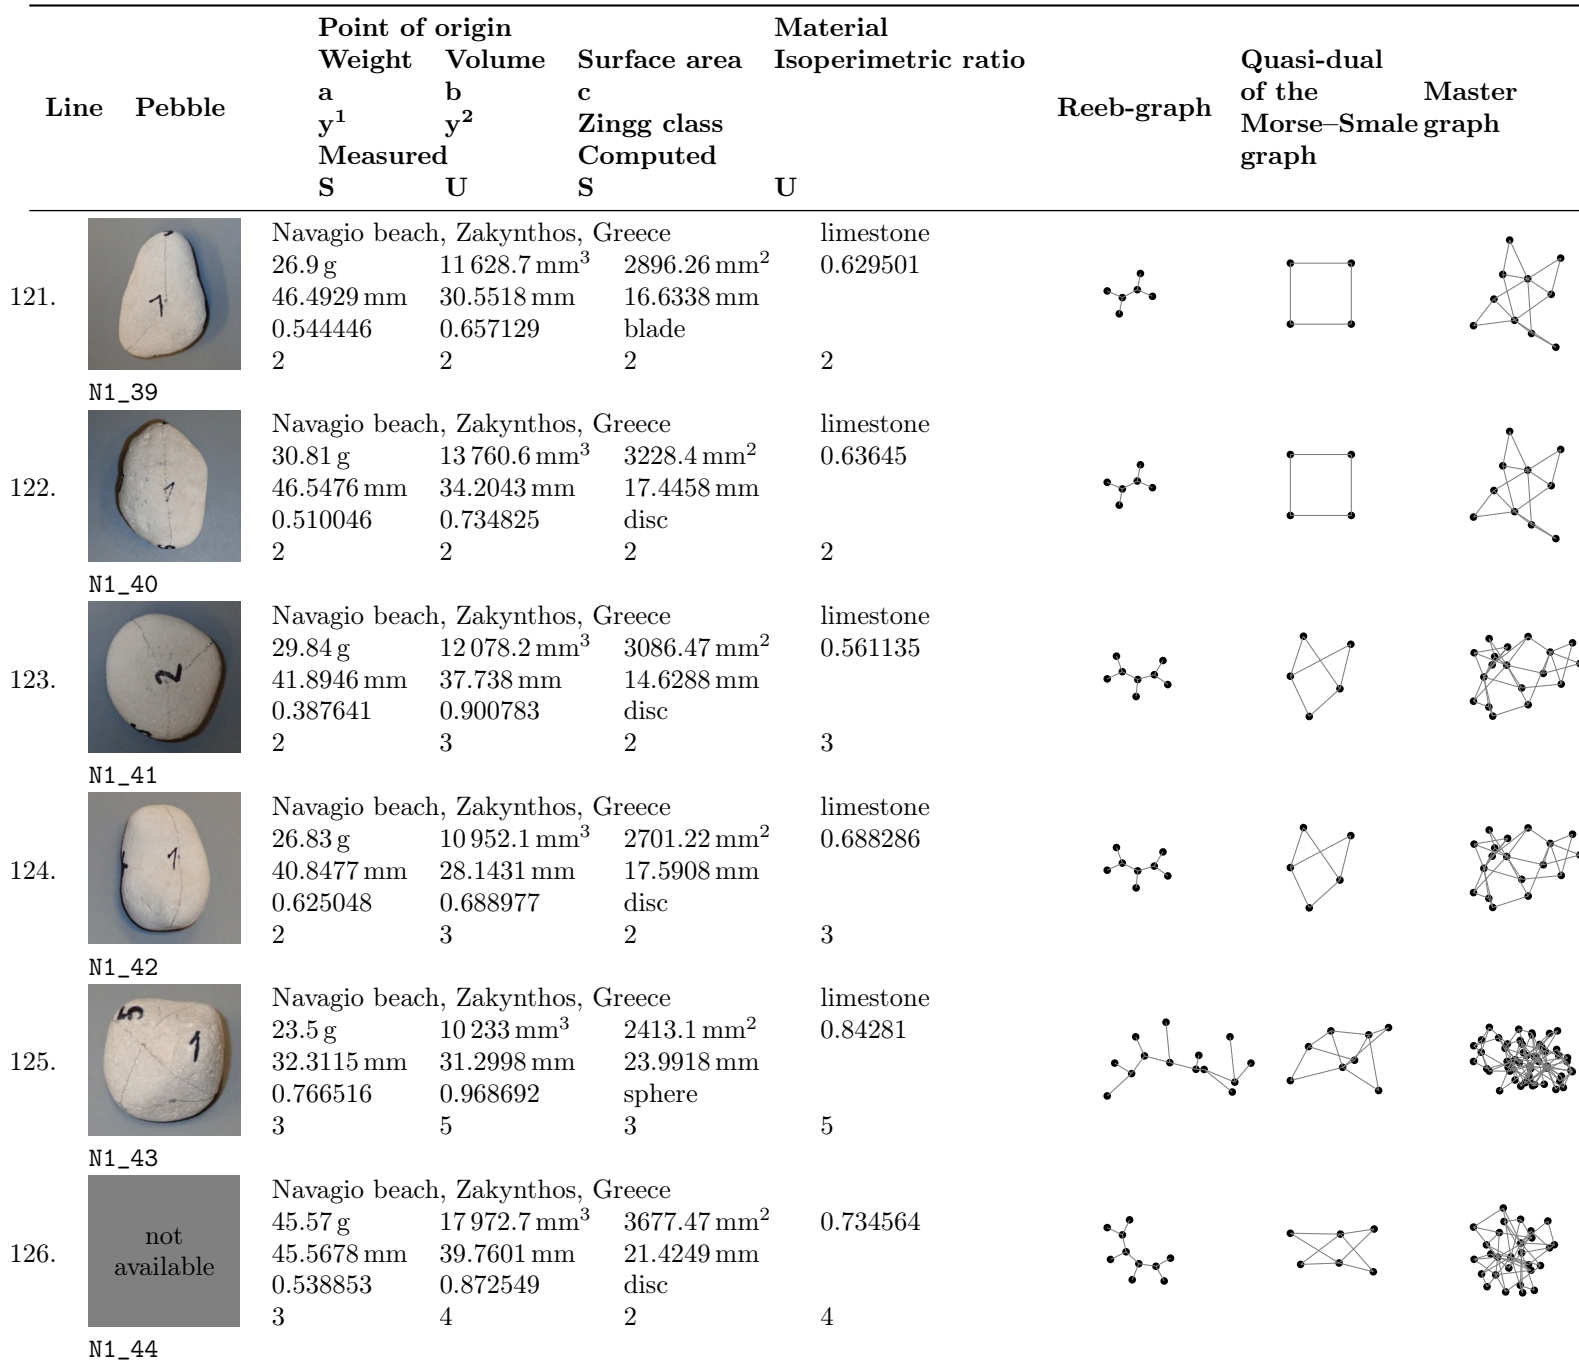   |
|      | N1_40                                                                               |                                                                            |                                                         |                                                     |                                |                                                                                       |                                                                                       |                                                                                       |
| 123. | 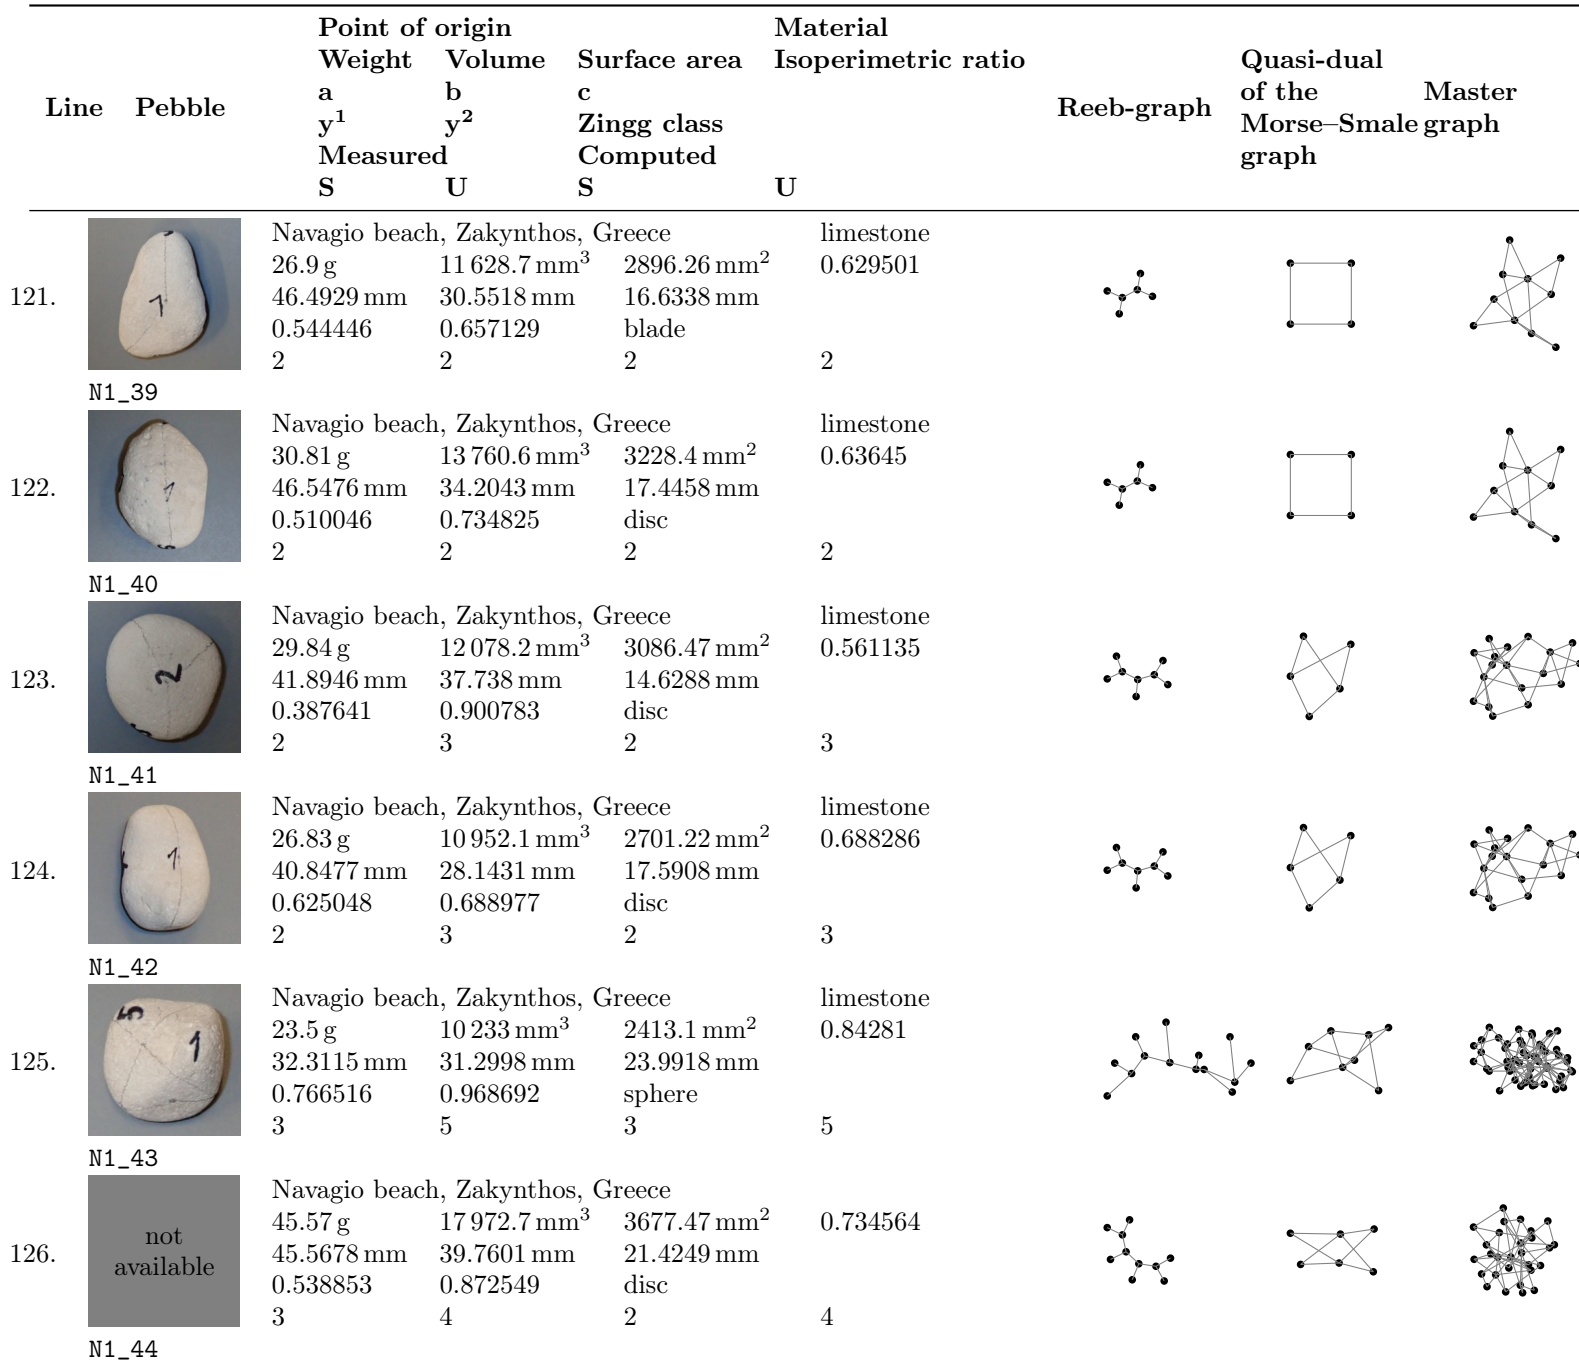   | Navagio beach, Zakynthos, Greece<br>29.84 g<br>41.8946 mm<br>0.387641<br>2 | 12 078.2 mm <sup>3</sup><br>37.738 mm<br>0.900783<br>3  | 3086.47 mm <sup>2</sup><br>14.6288 mm<br>disc<br>2  | limestone<br>0.561135<br><br>3 | 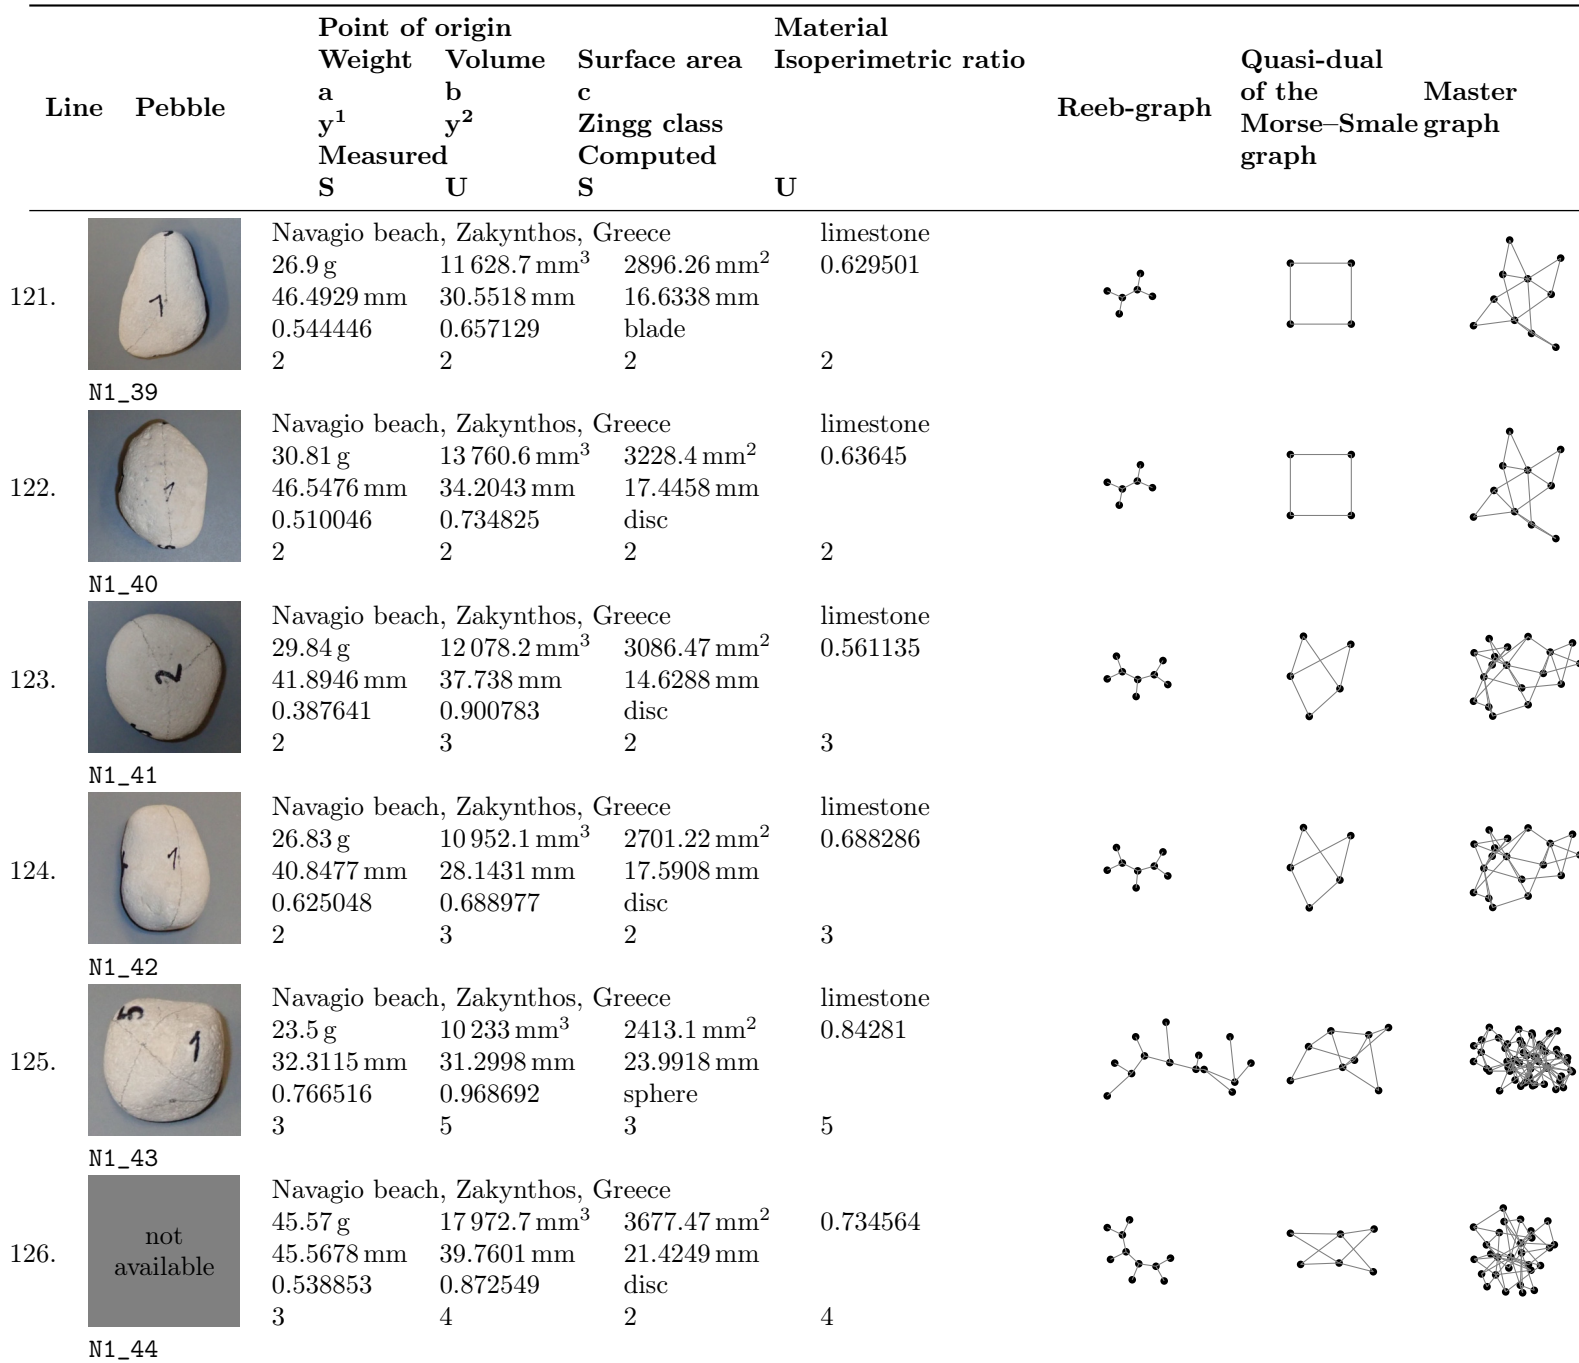   | 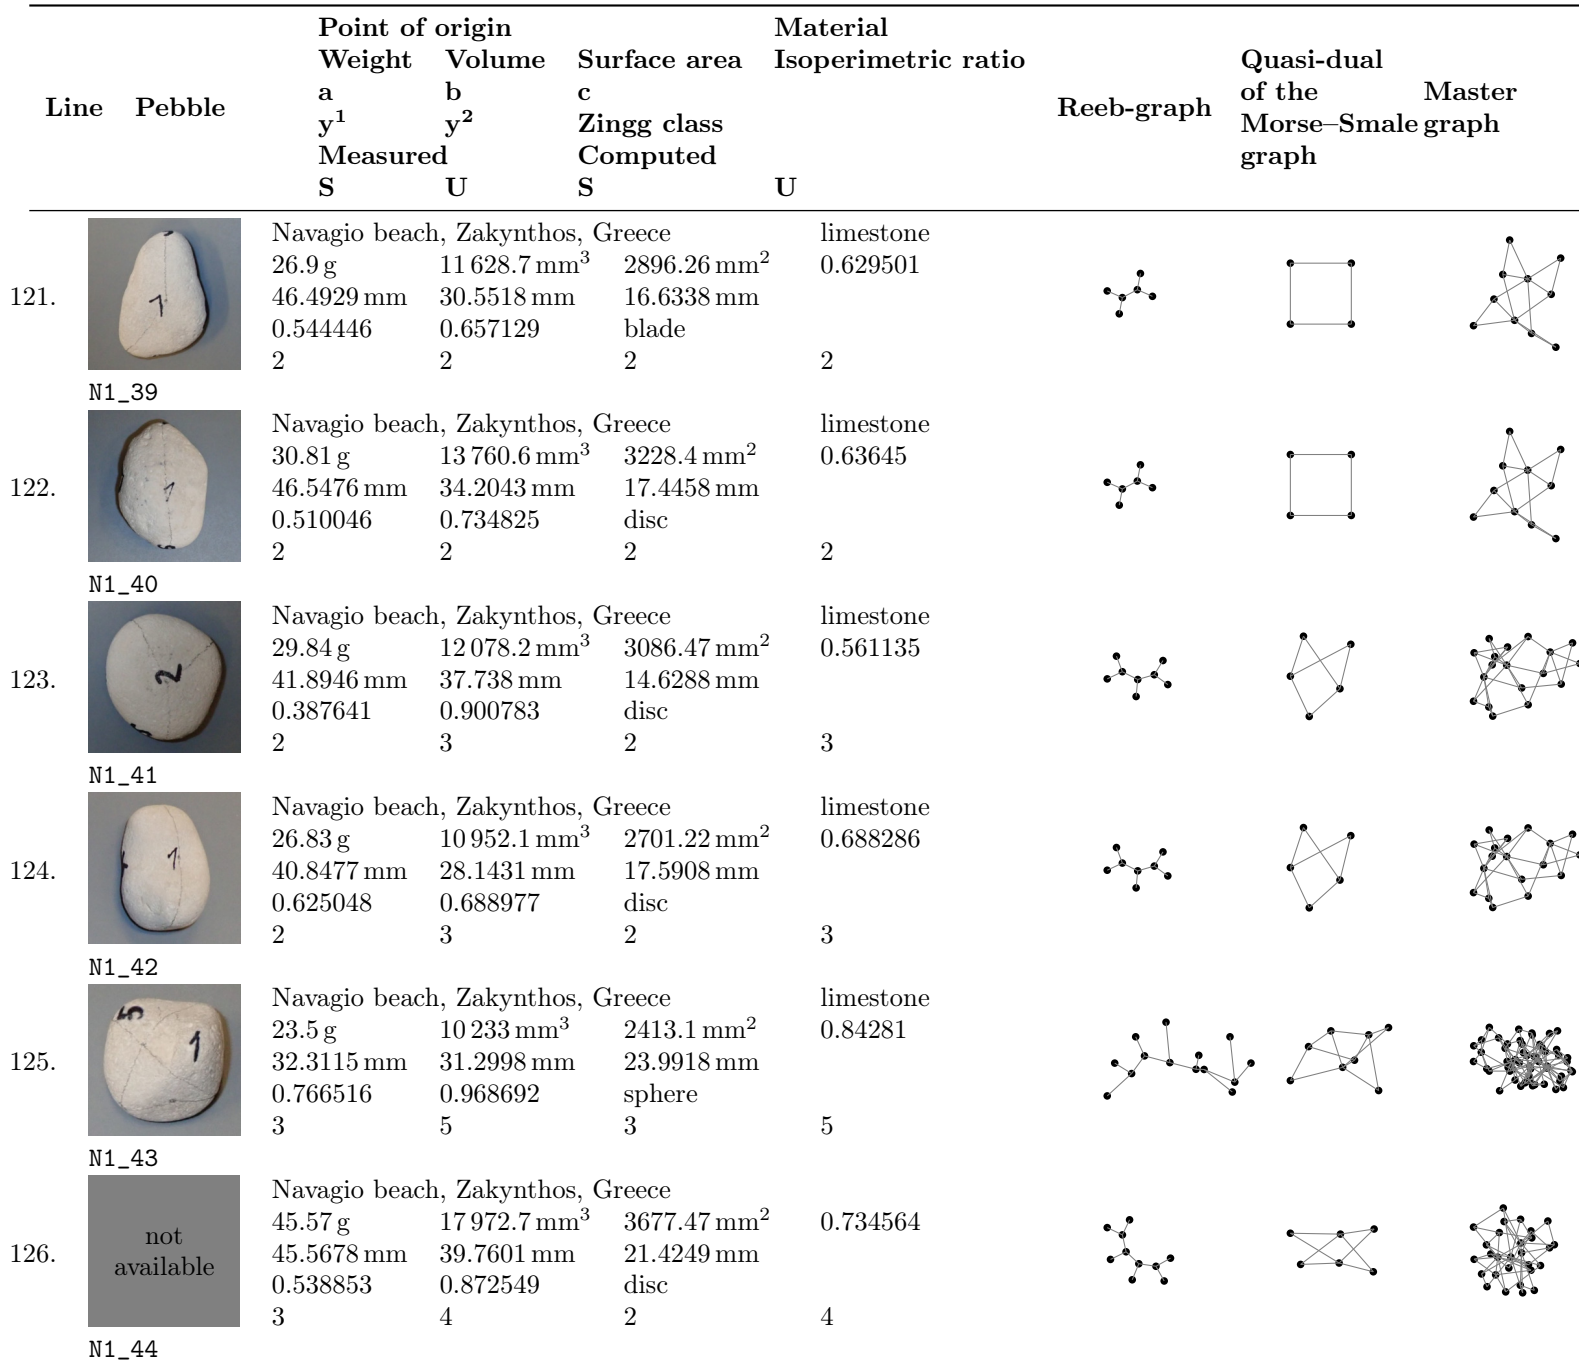   | 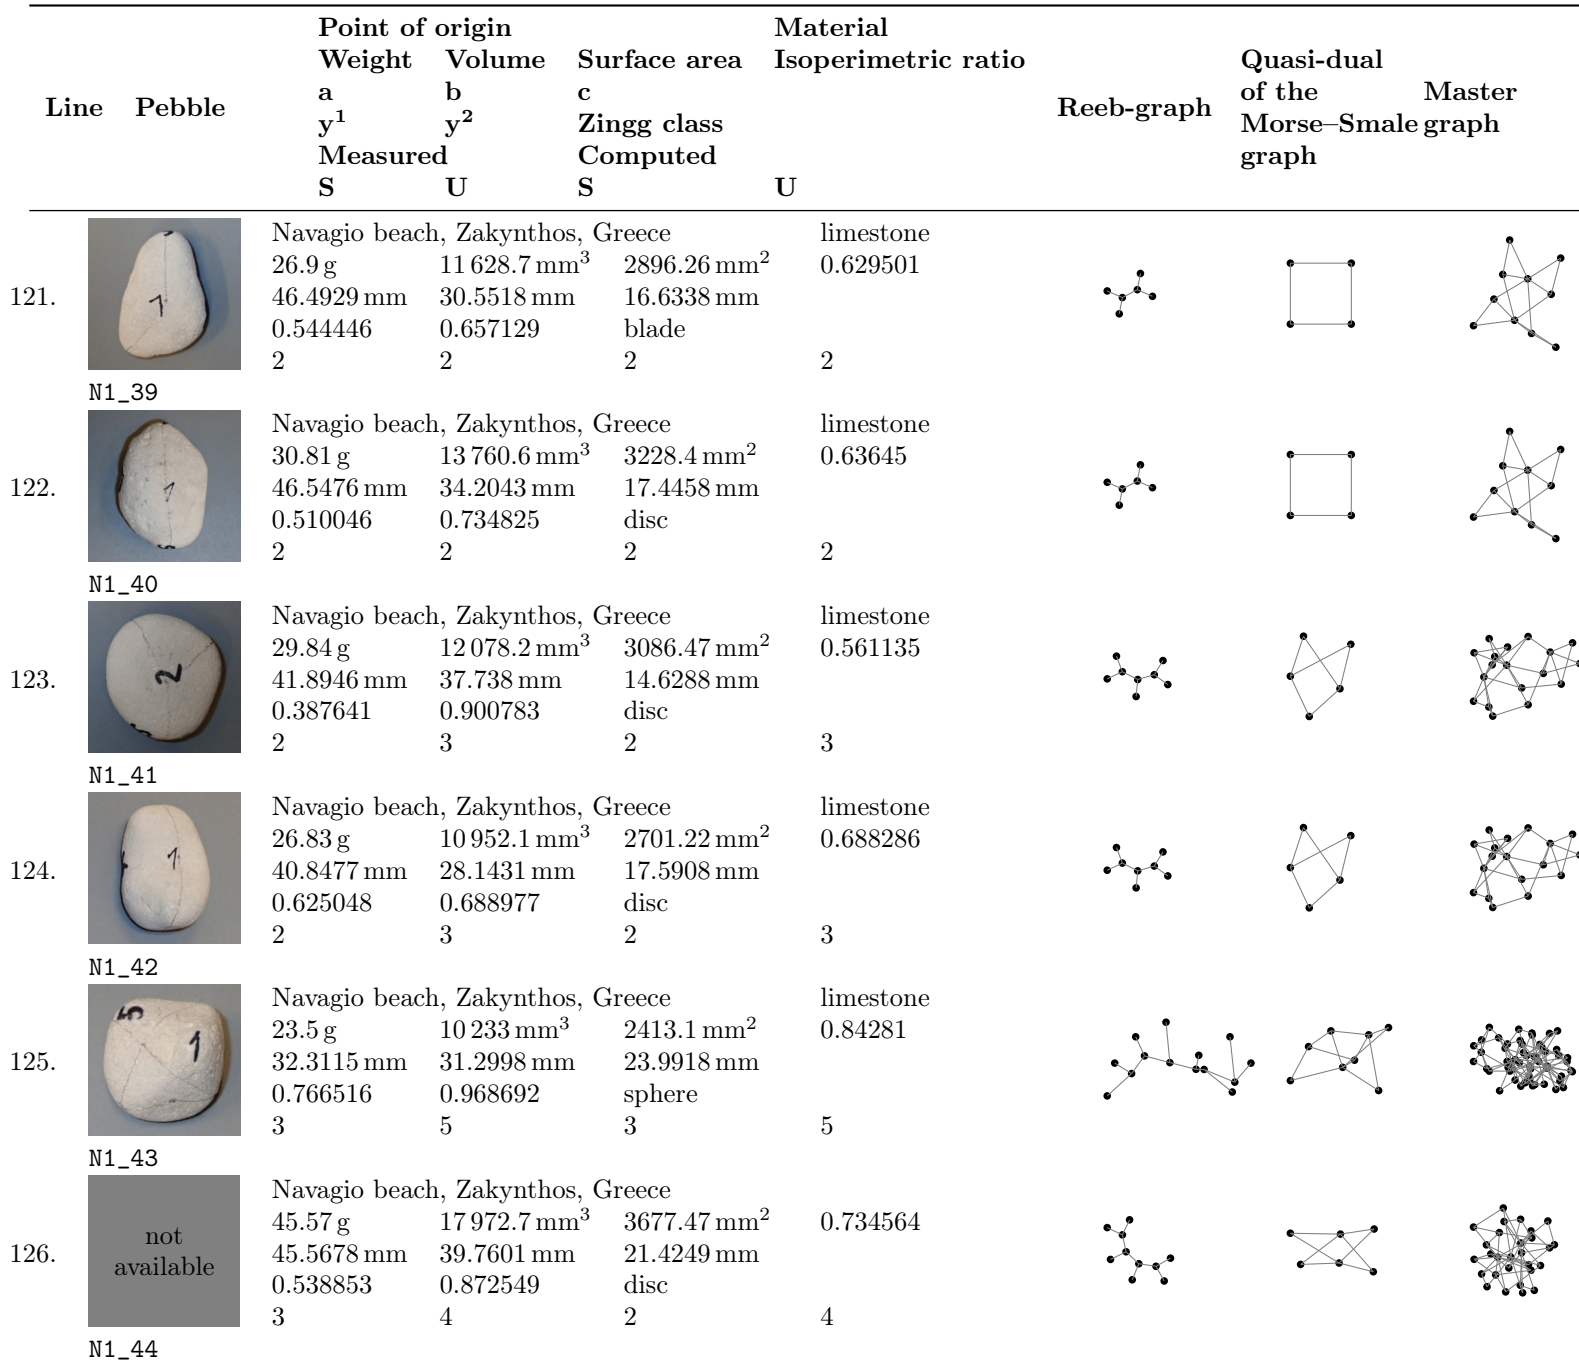   |
|      | N1_41                                                                               |                                                                            |                                                         |                                                     |                                |                                                                                       |                                                                                       |                                                                                       |
| 124. | 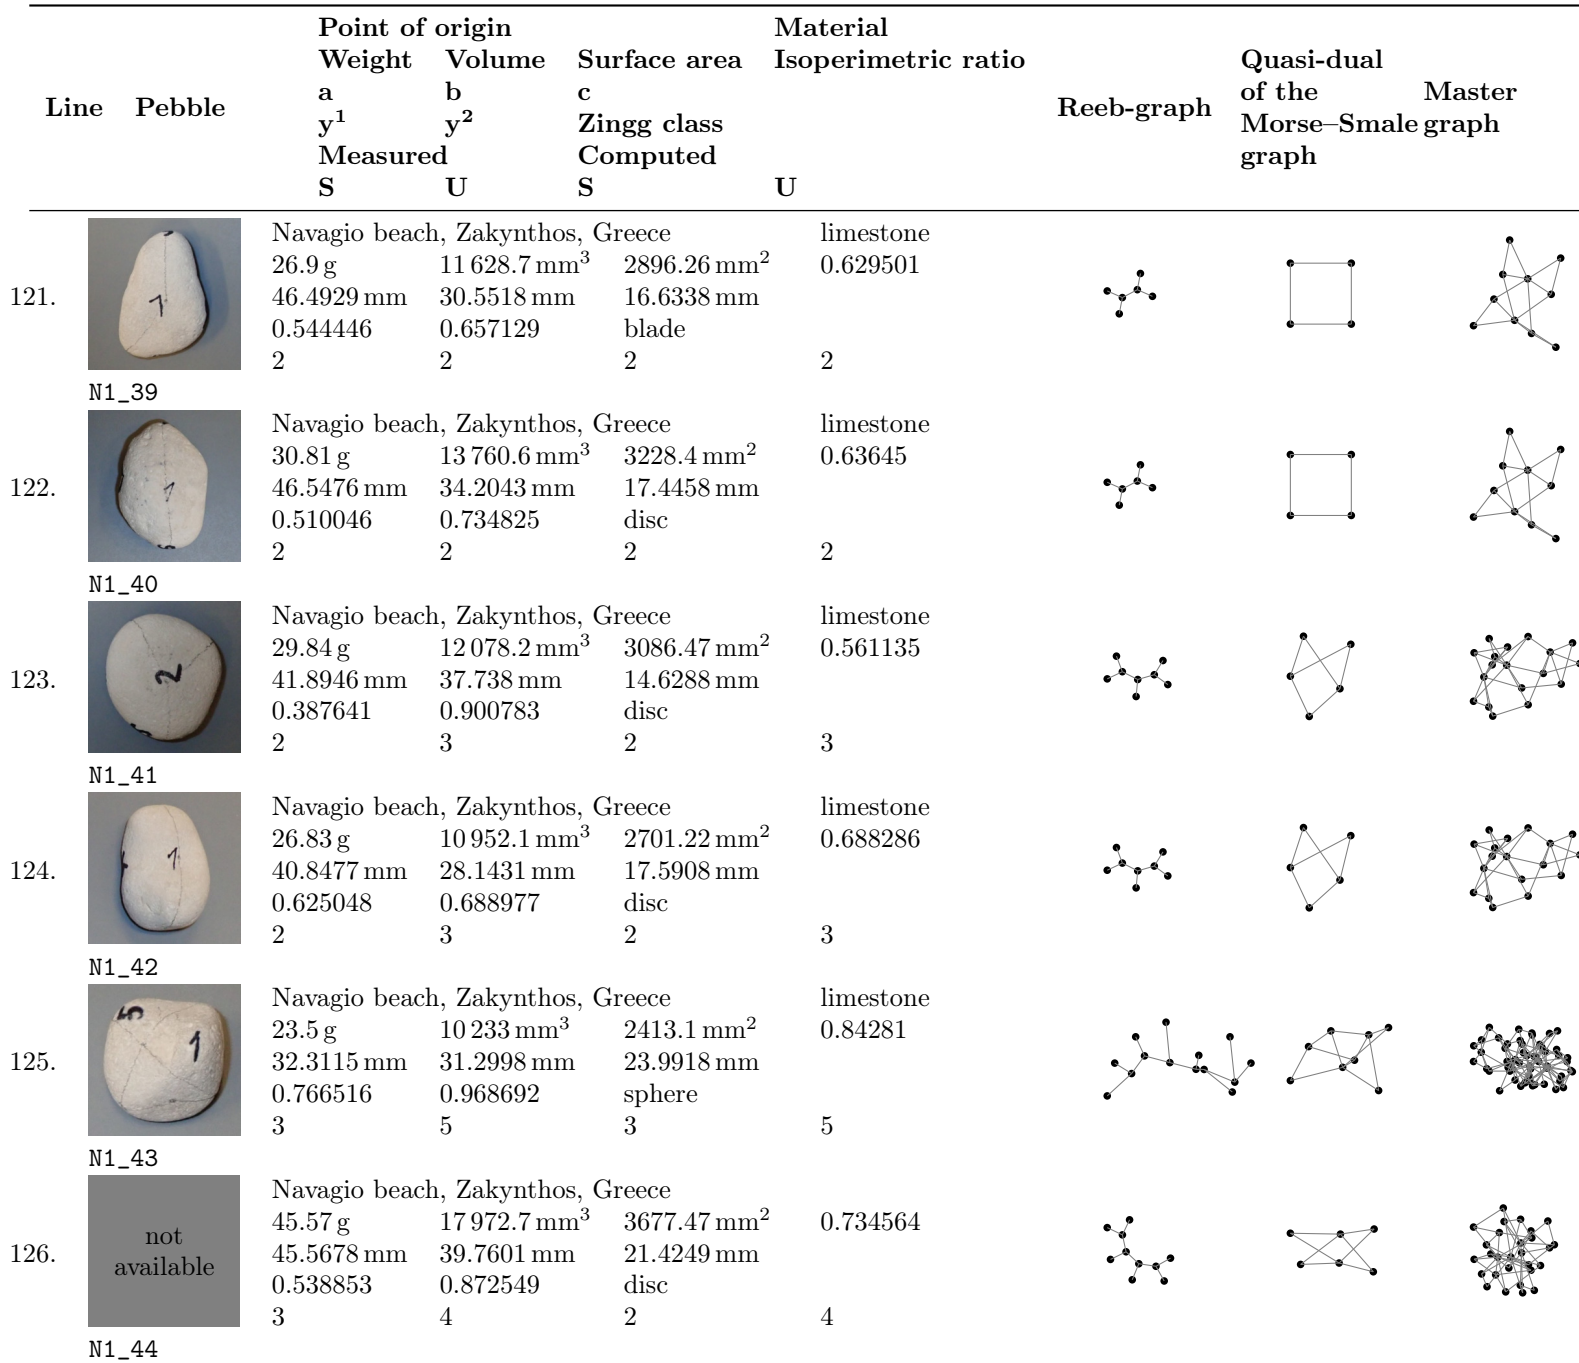  | Navagio beach, Zakynthos, Greece<br>26.83 g<br>40.8477 mm<br>0.625048<br>2 | 10 952.1 mm <sup>3</sup><br>28.1431 mm<br>0.688977<br>3 | 2701.22 mm <sup>2</sup><br>17.5908 mm<br>disc<br>2  | limestone<br>0.688286<br><br>3 | 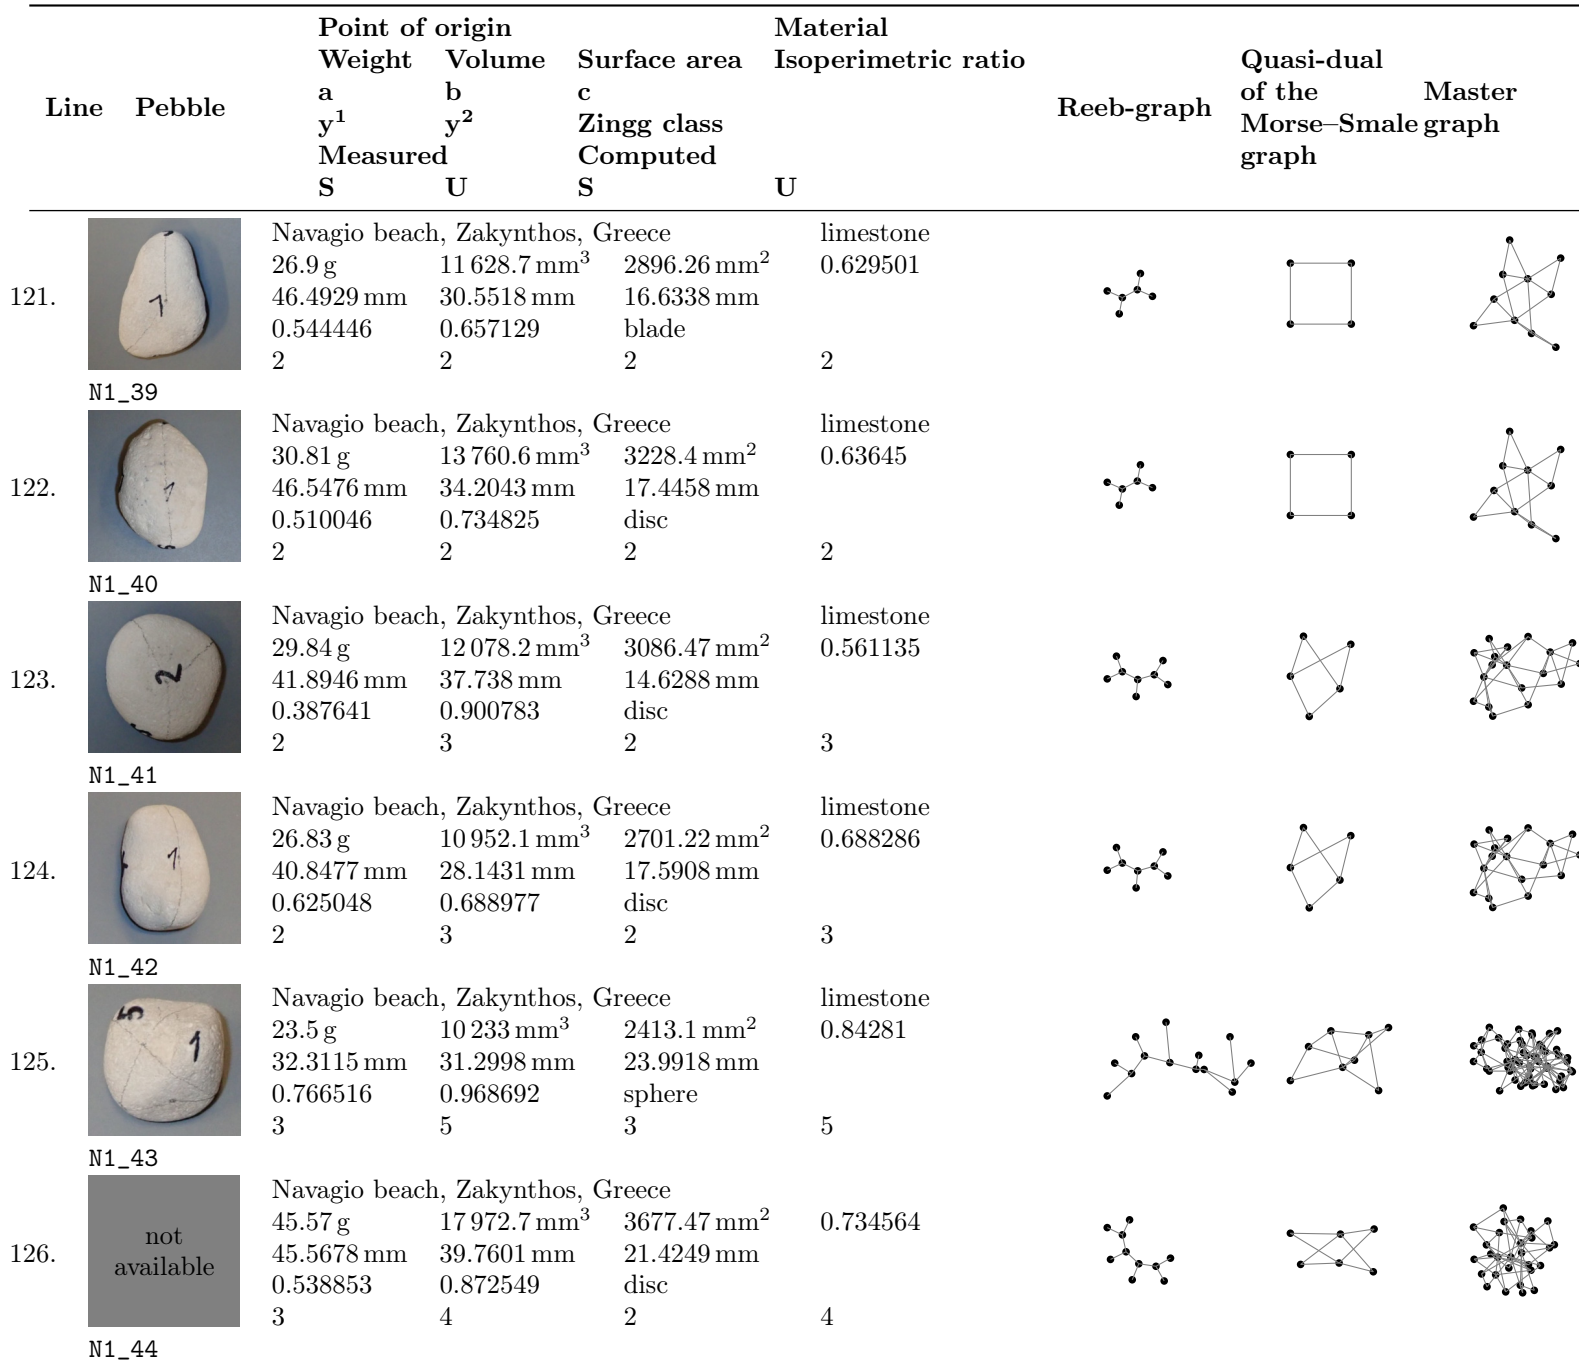  | 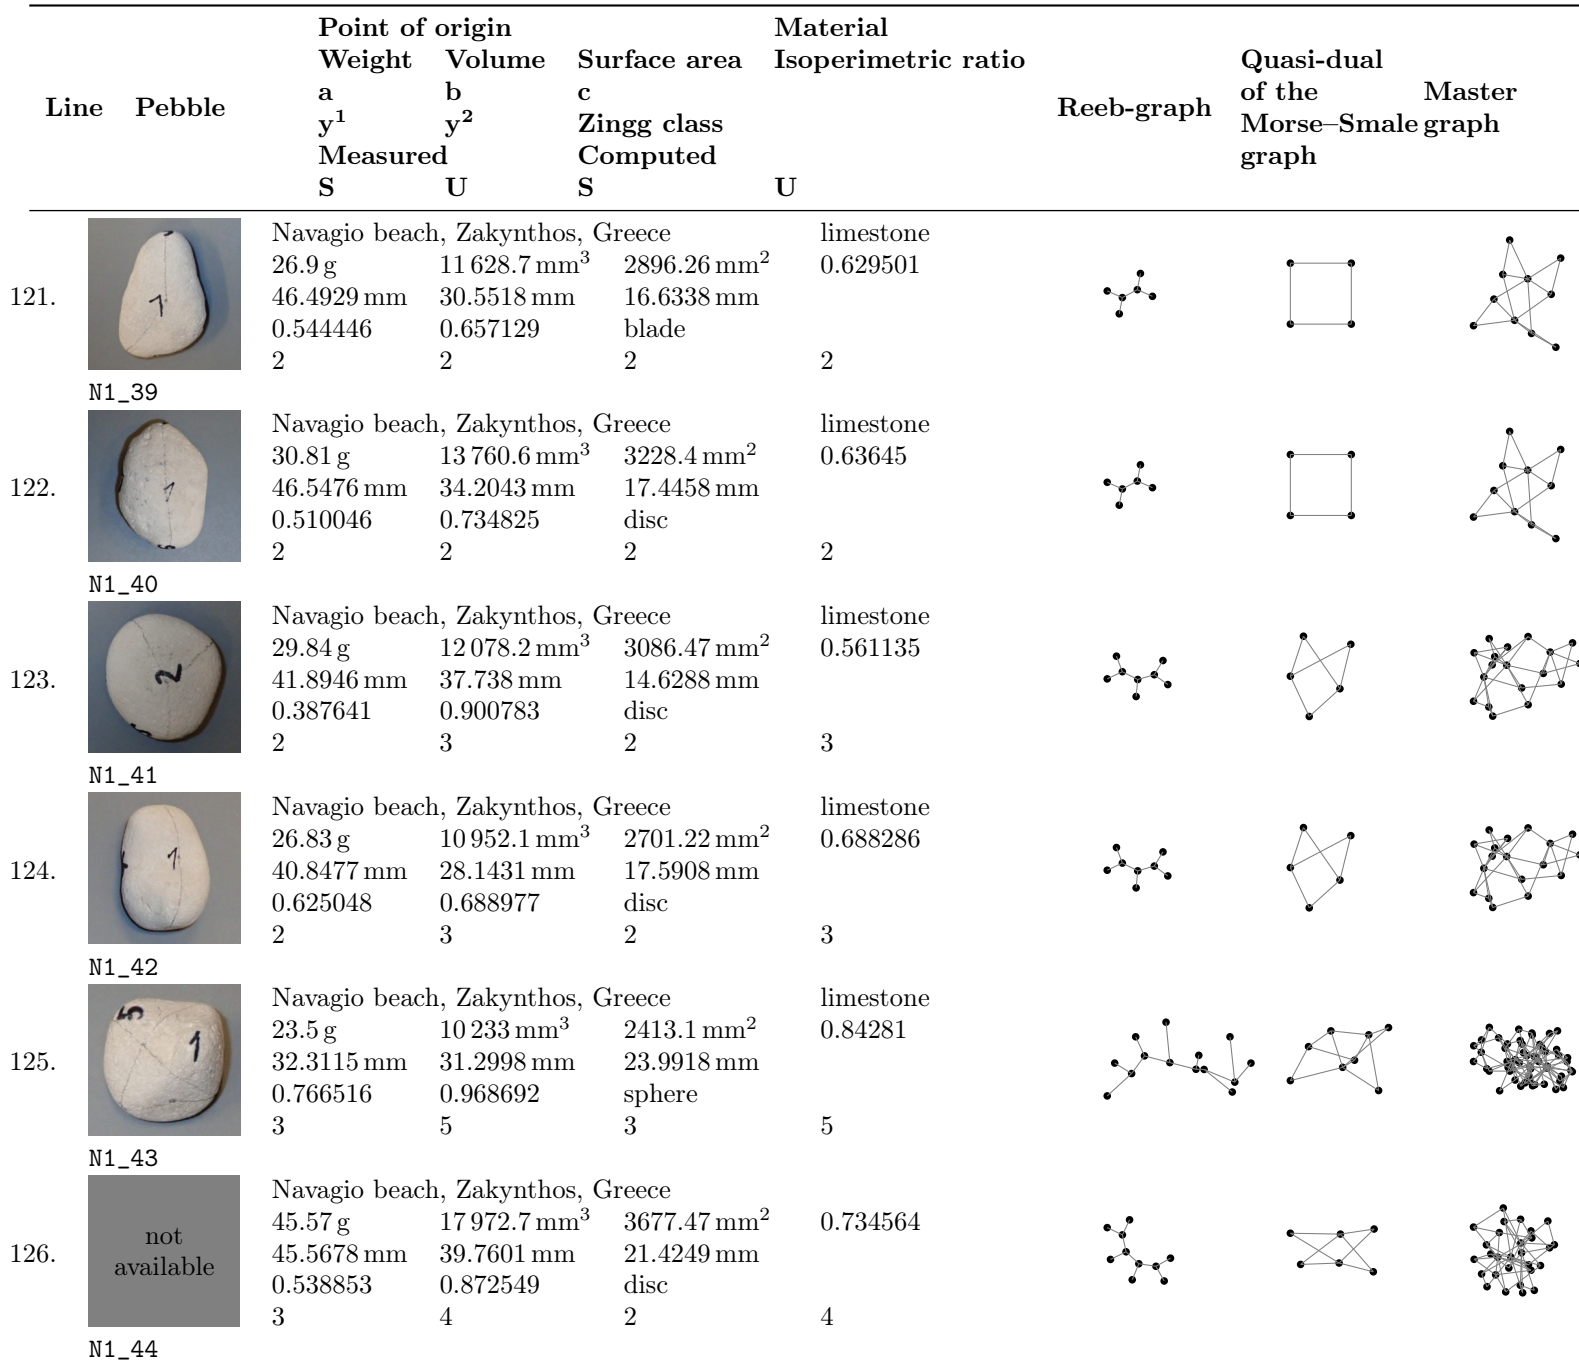  | 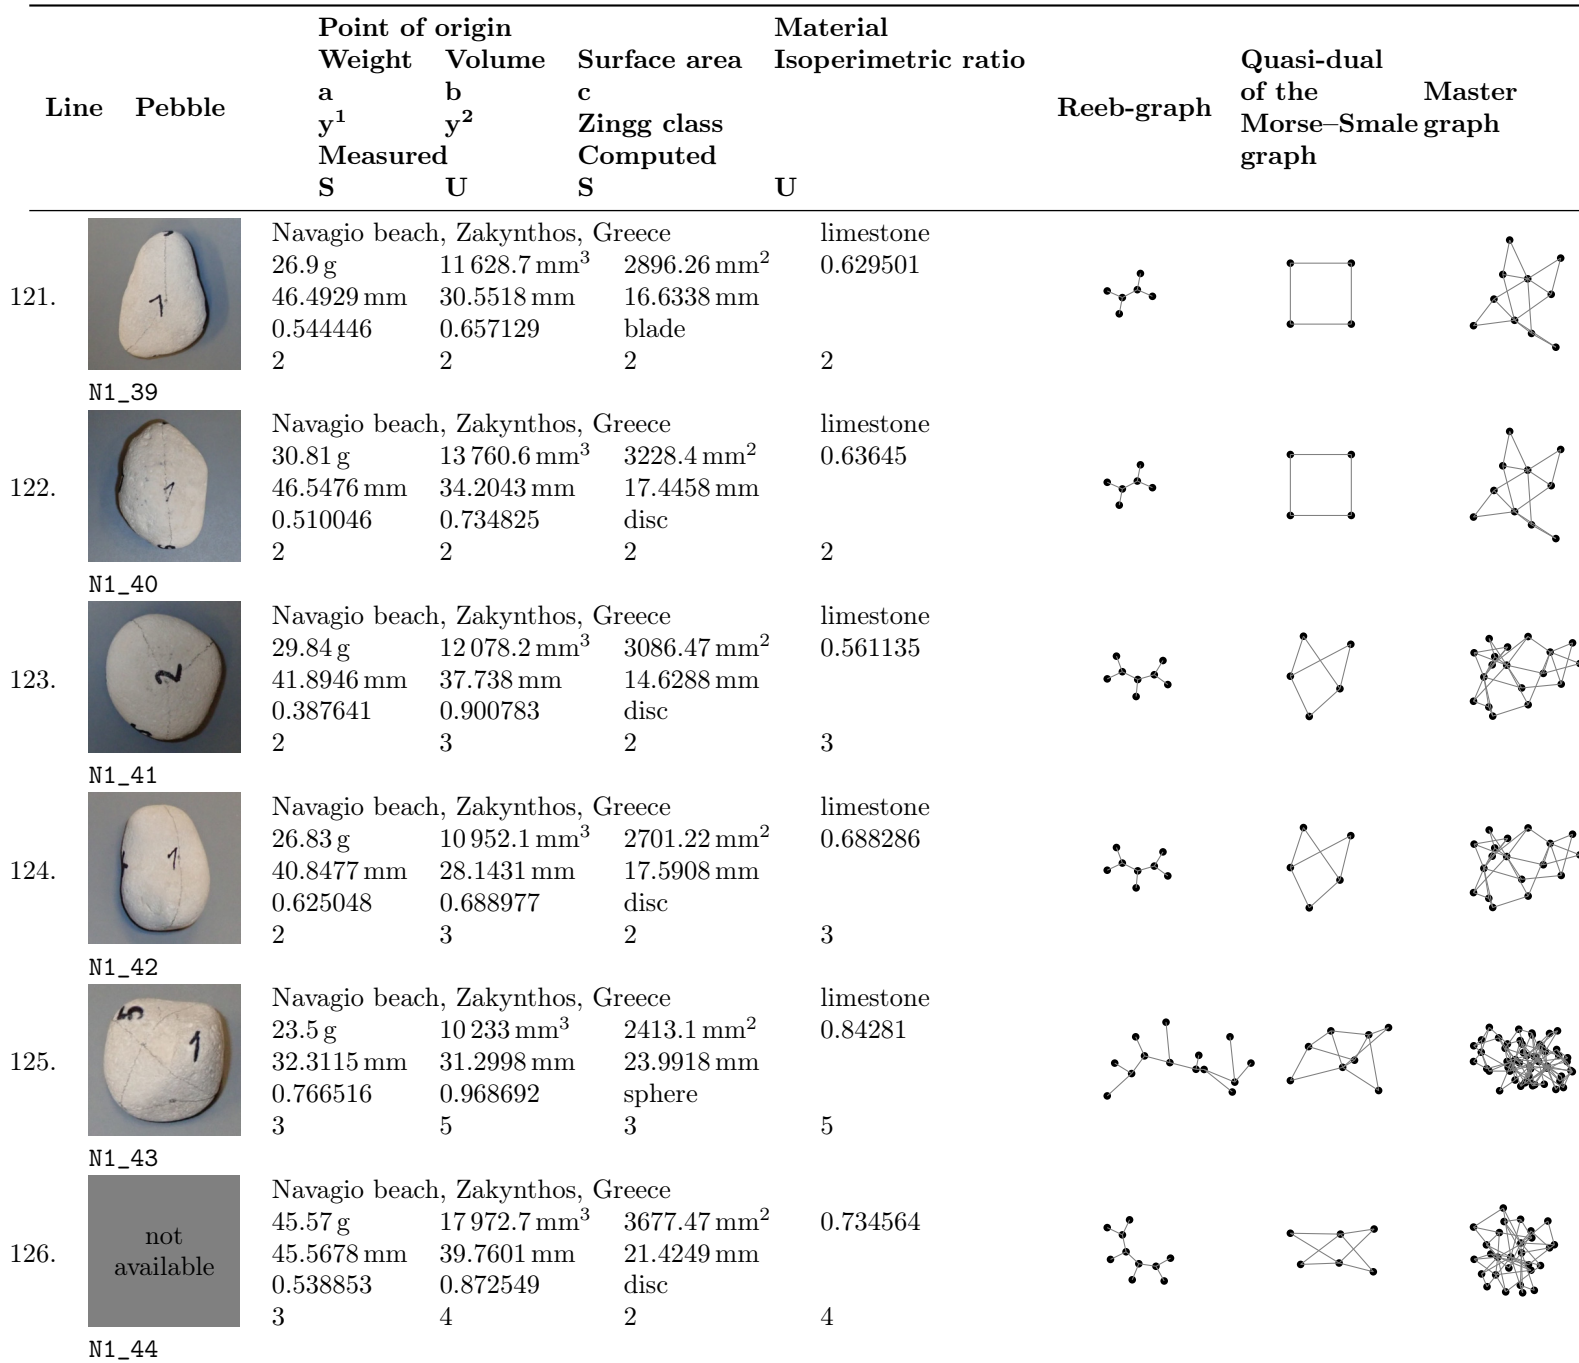  |
|      | N1_42                                                                               |                                                                            |                                                         |                                                     |                                |                                                                                       |                                                                                       |                                                                                       |
| 125. | 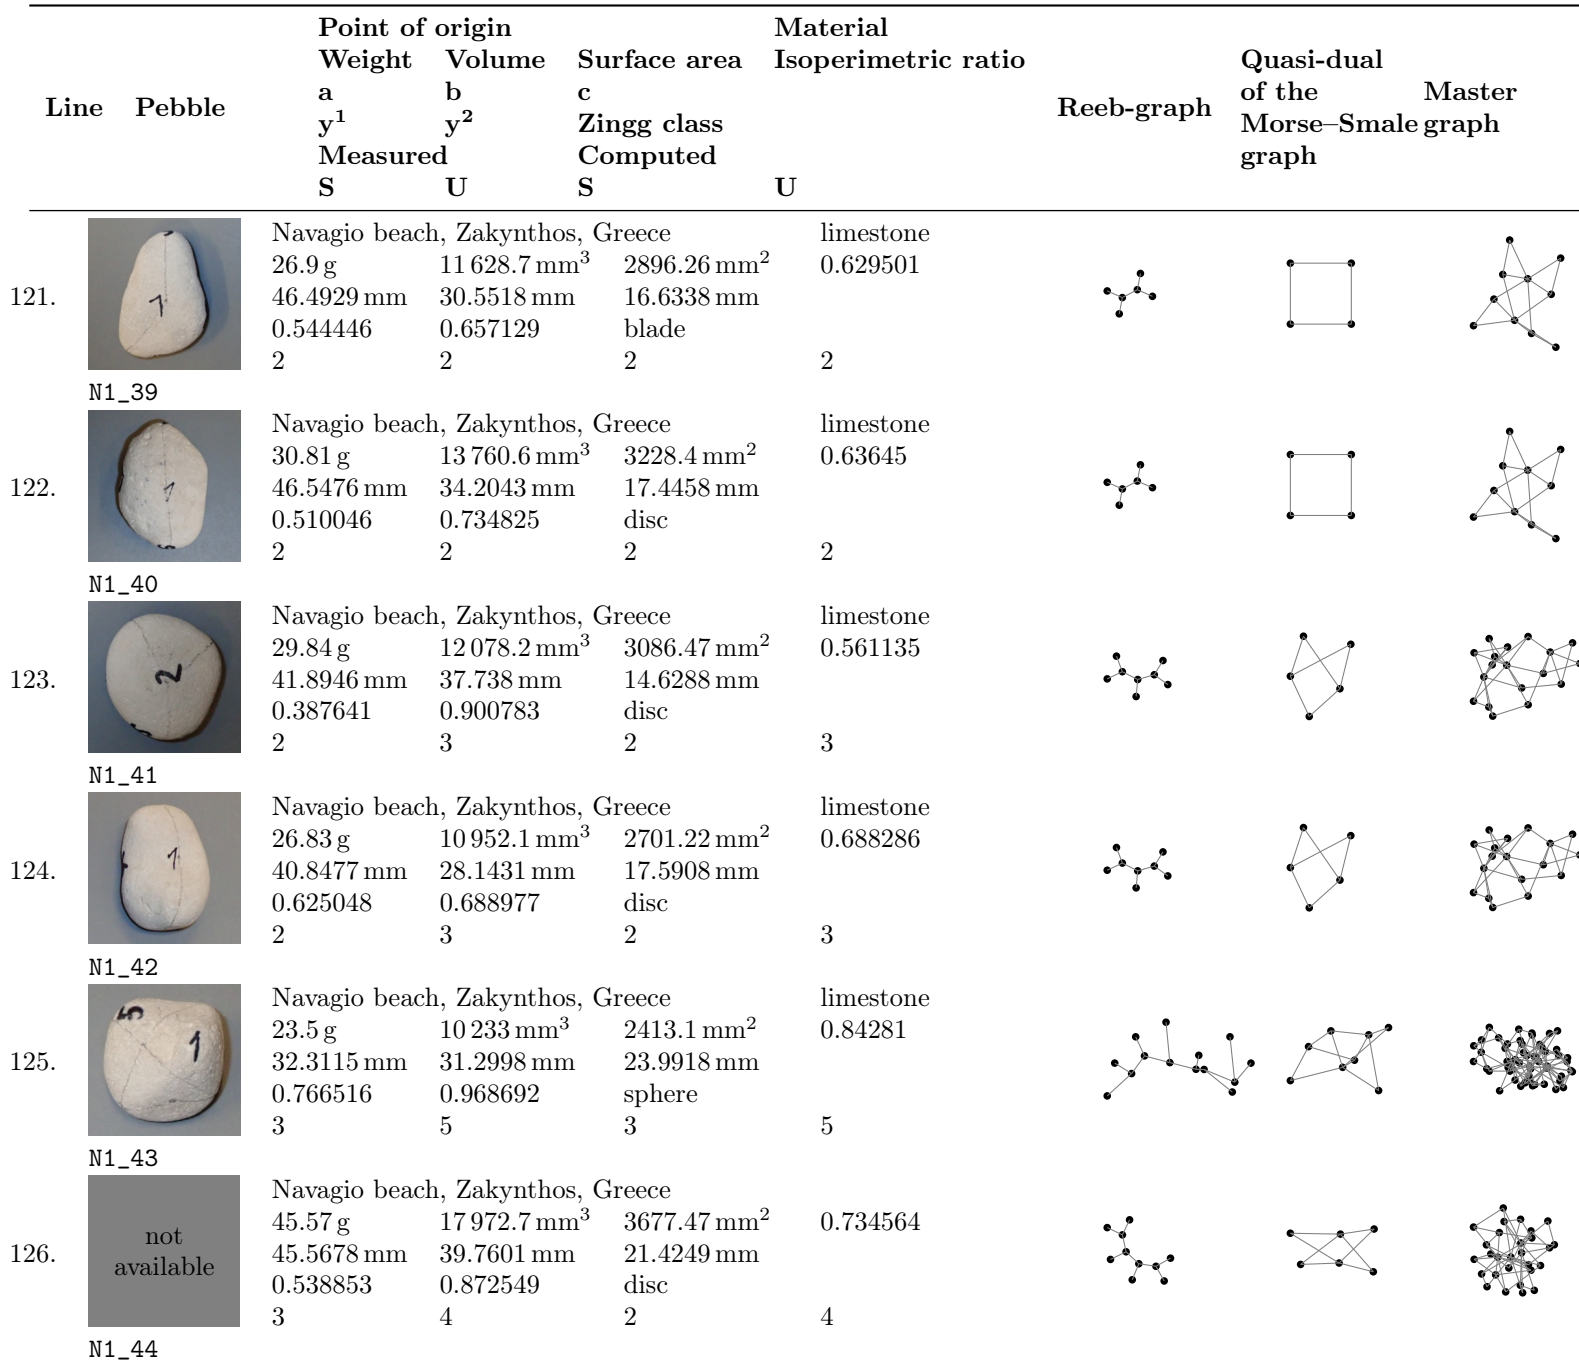 | Navagio beach, Zakynthos, Greece<br>23.5 g<br>32.3115 mm<br>0.766516<br>3  | 10 233 mm <sup>3</sup><br>31.2998 mm<br>0.968692<br>5   | 2413.1 mm <sup>2</sup><br>23.9918 mm<br>sphere<br>3 | limestone<br>0.84281<br><br>5  | 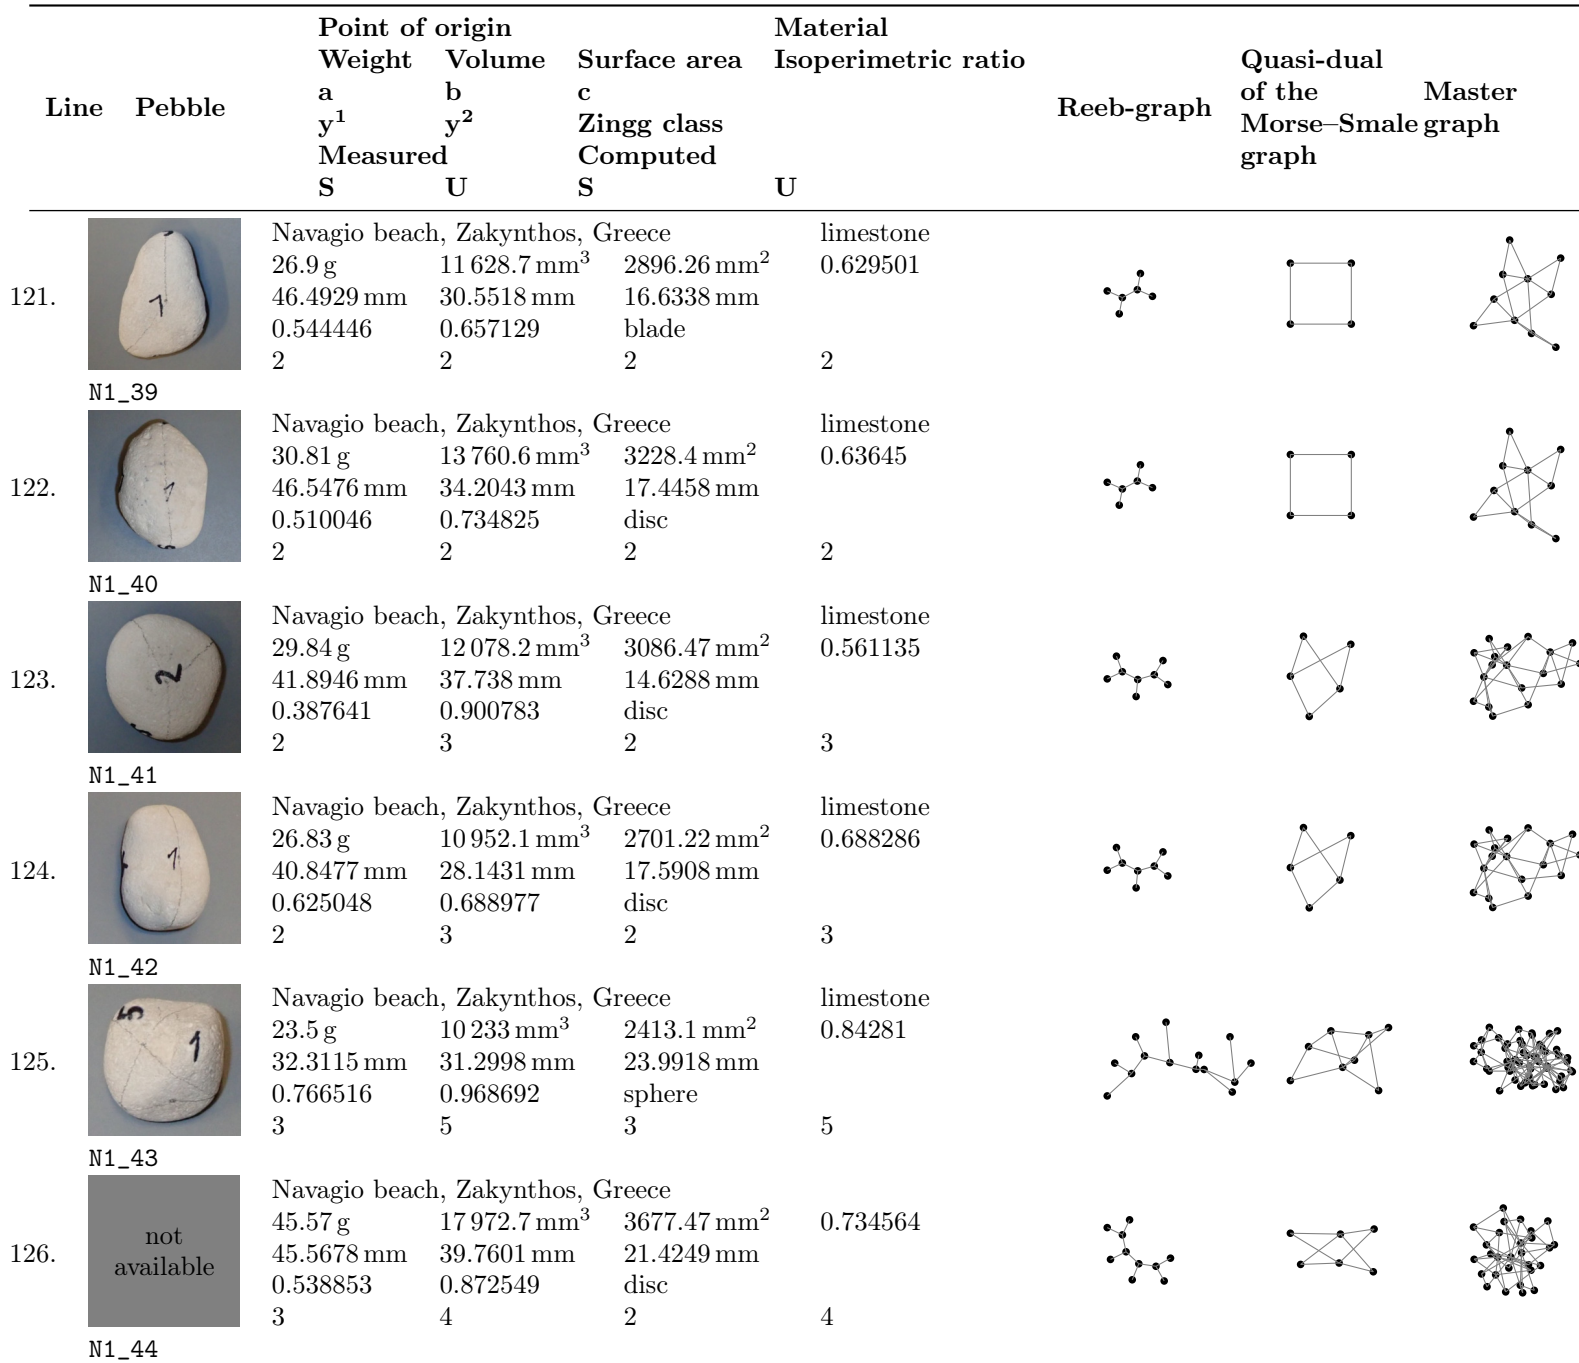 | 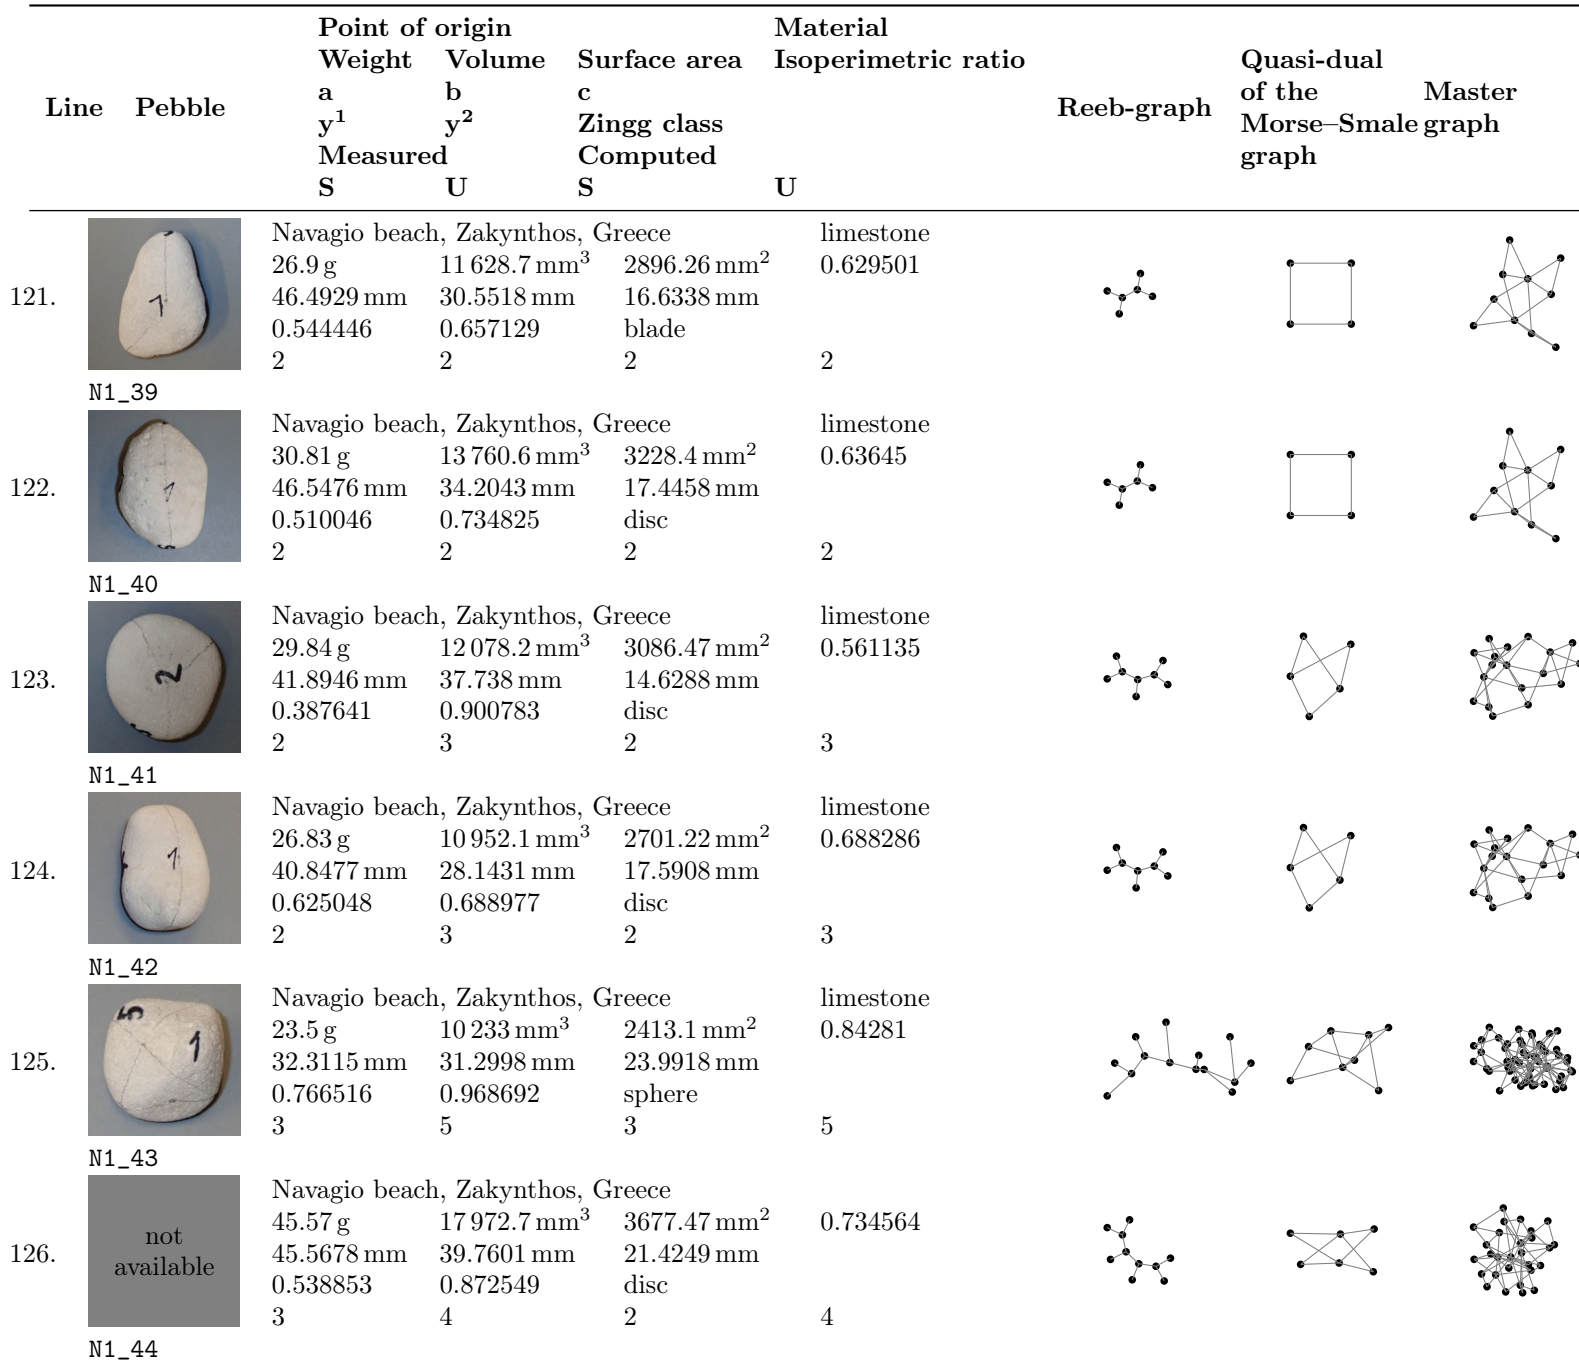 | 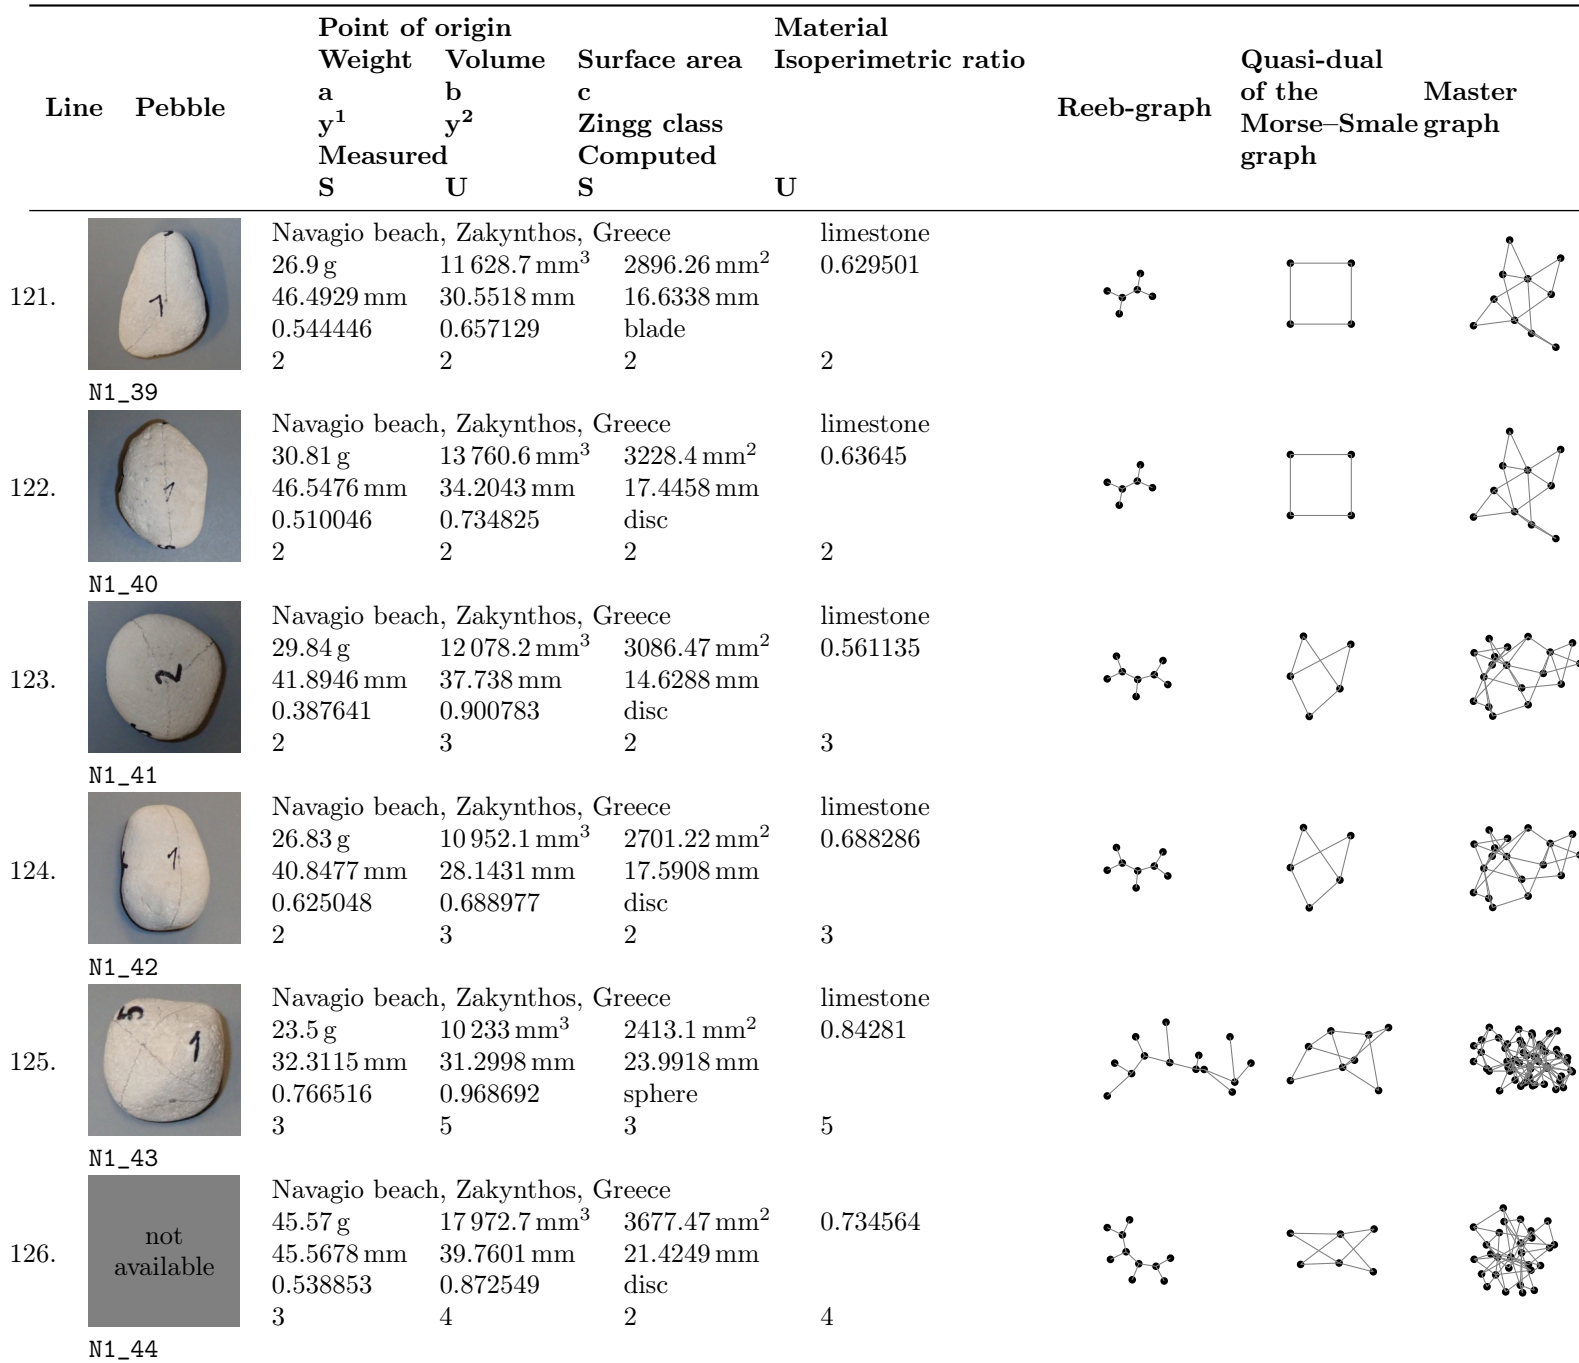 |
|      | N1_43                                                                               |                                                                            |                                                         |                                                     |                                |                                                                                       |                                                                                       |                                                                                       |
| 126. | 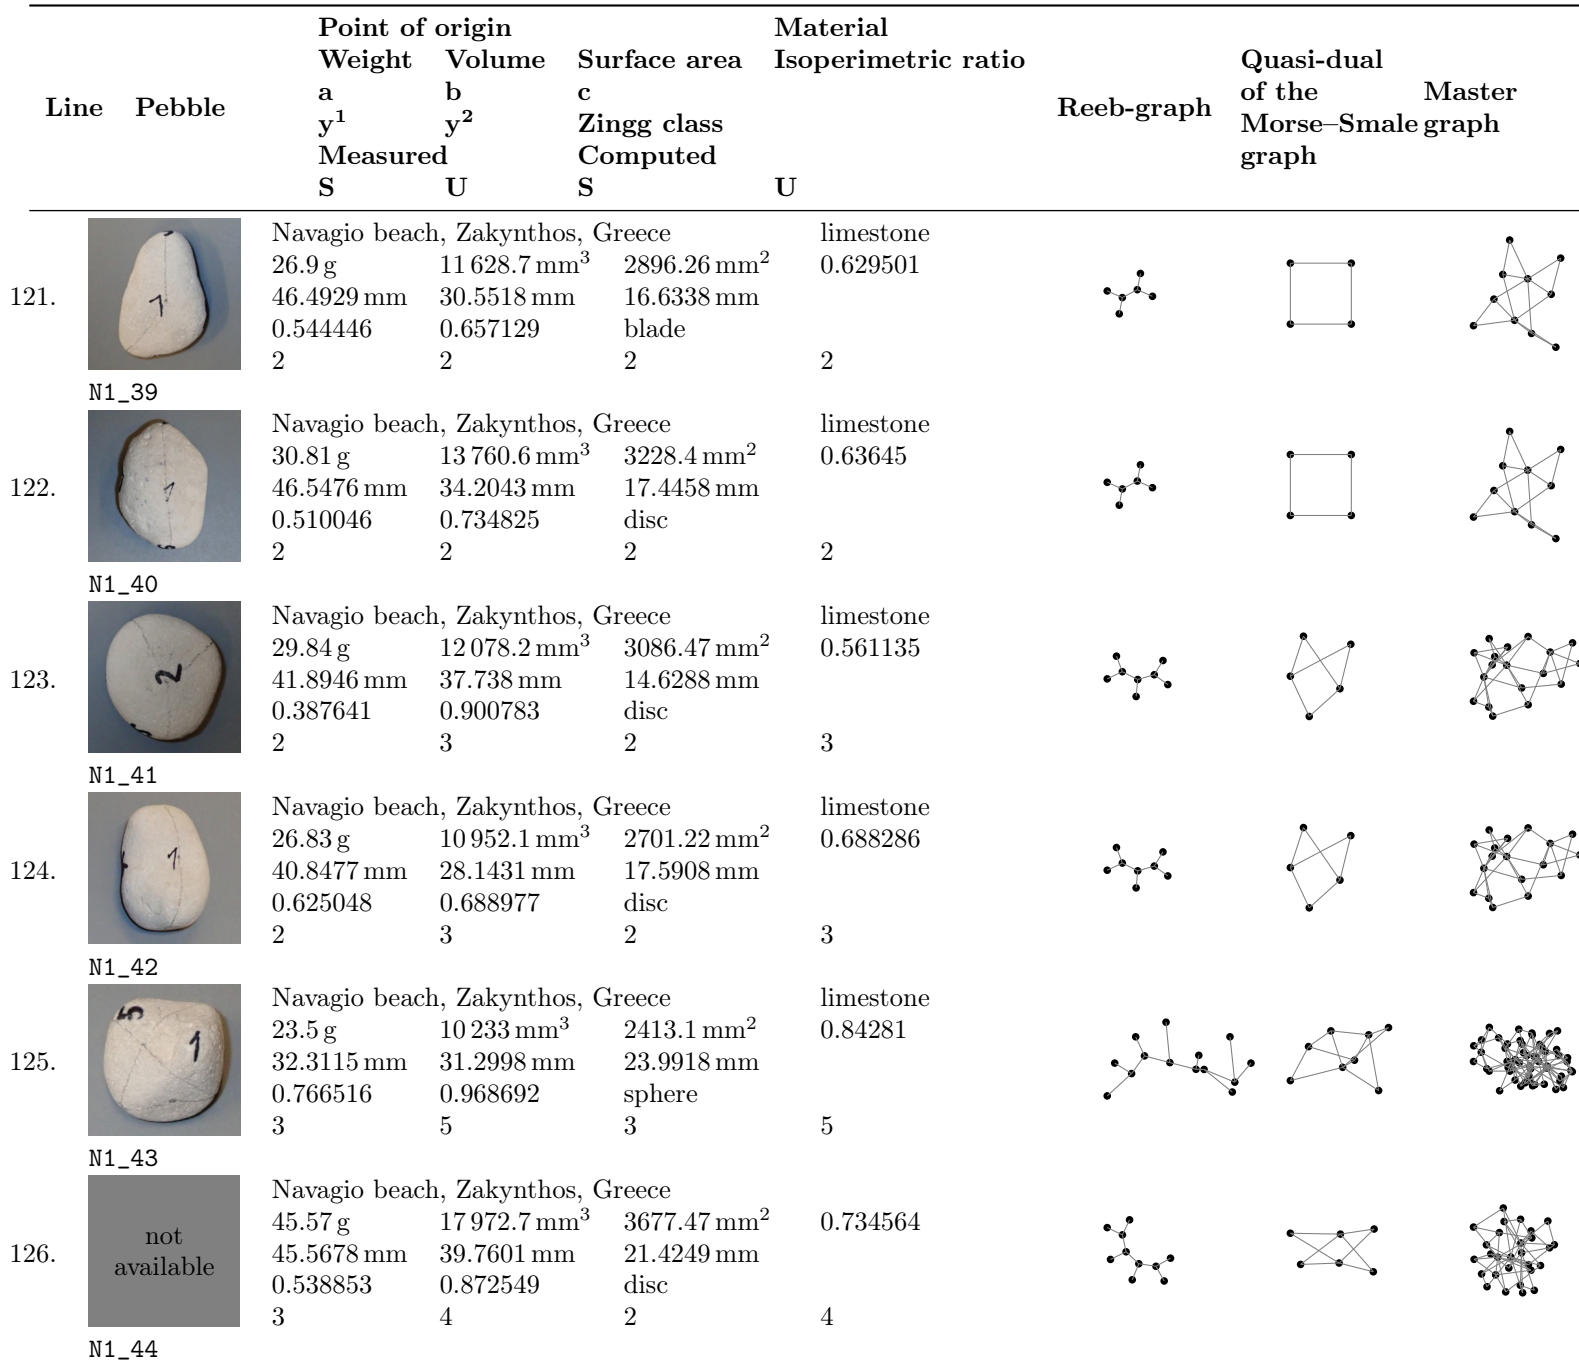 | Navagio beach, Zakynthos, Greece<br>45.57 g<br>45.5678 mm<br>0.538853<br>3 | 17 972.7 mm <sup>3</sup><br>39.7601 mm<br>0.872549<br>4 | 3677.47 mm <sup>2</sup><br>21.4249 mm<br>disc<br>2  | limestone<br>0.734564<br><br>4 | 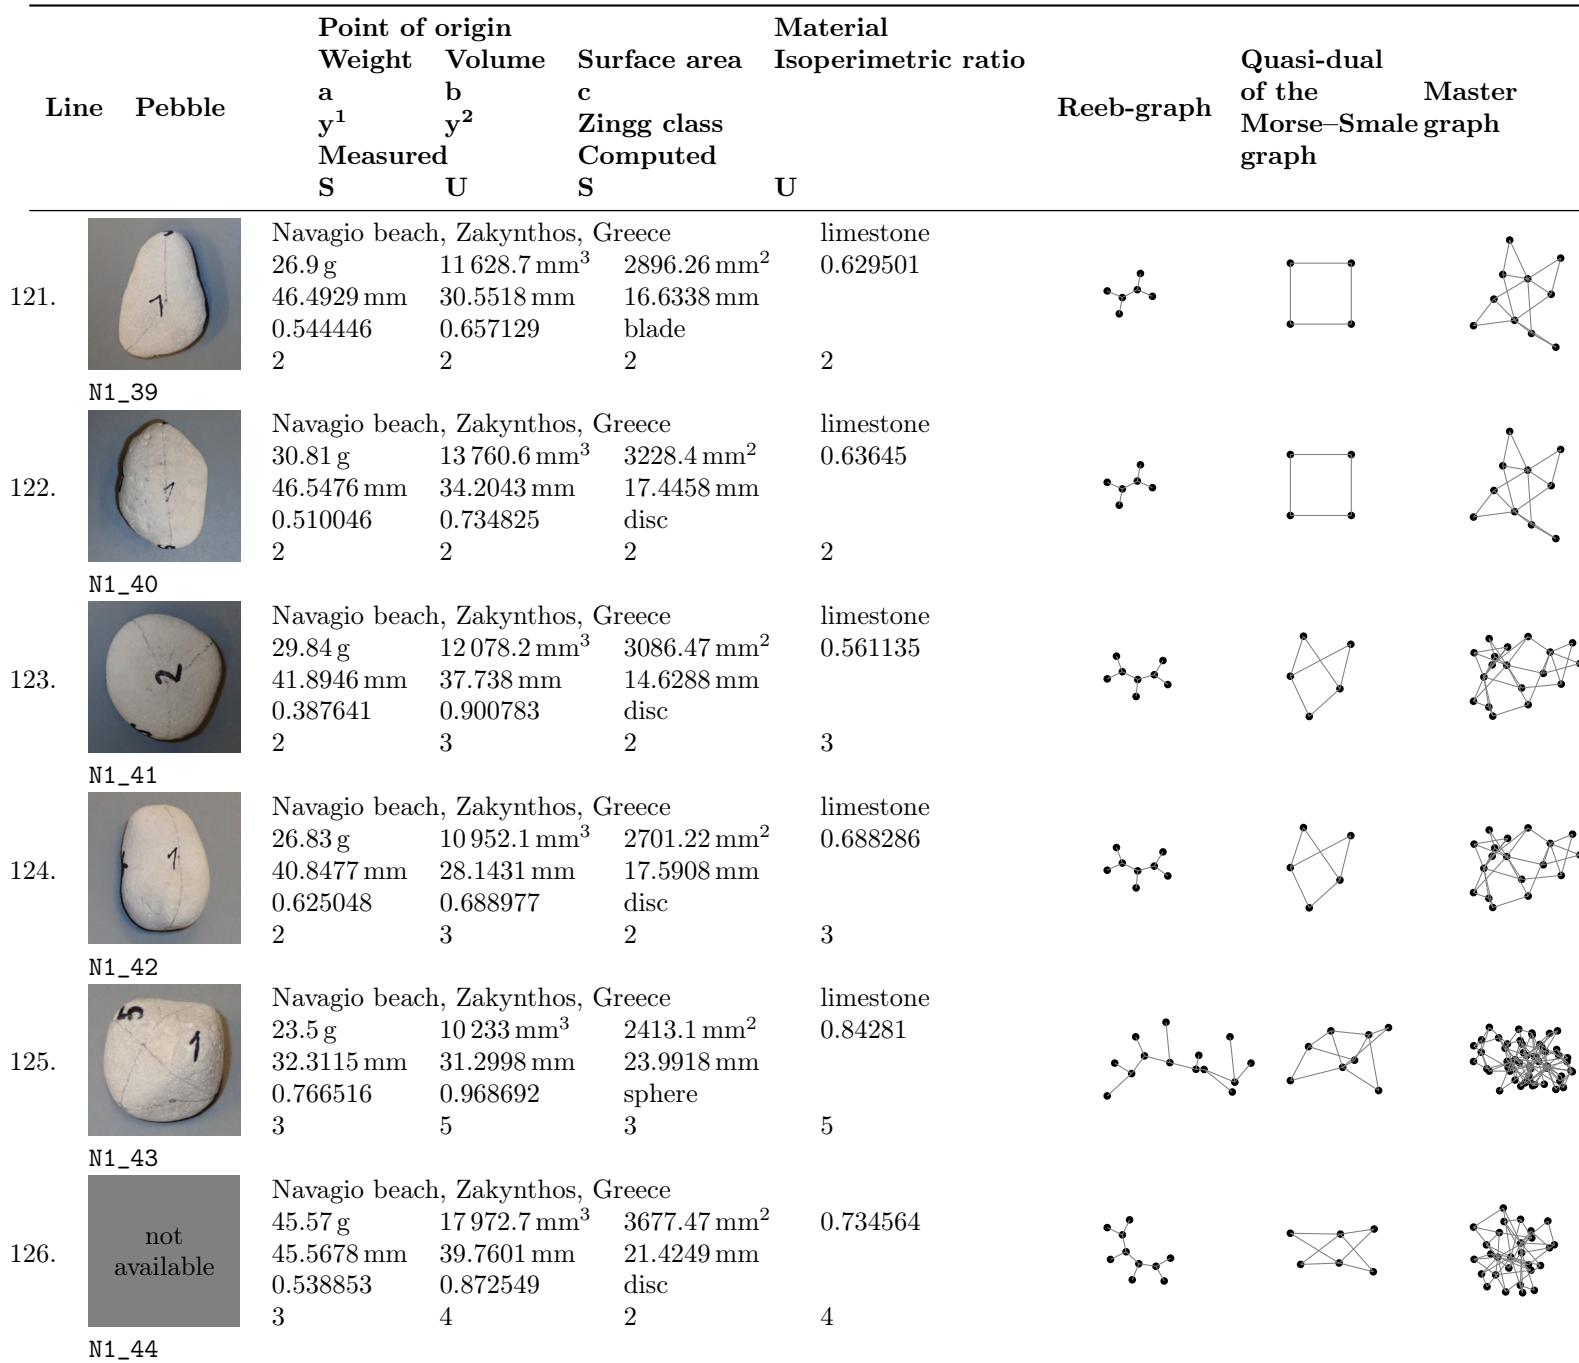 | 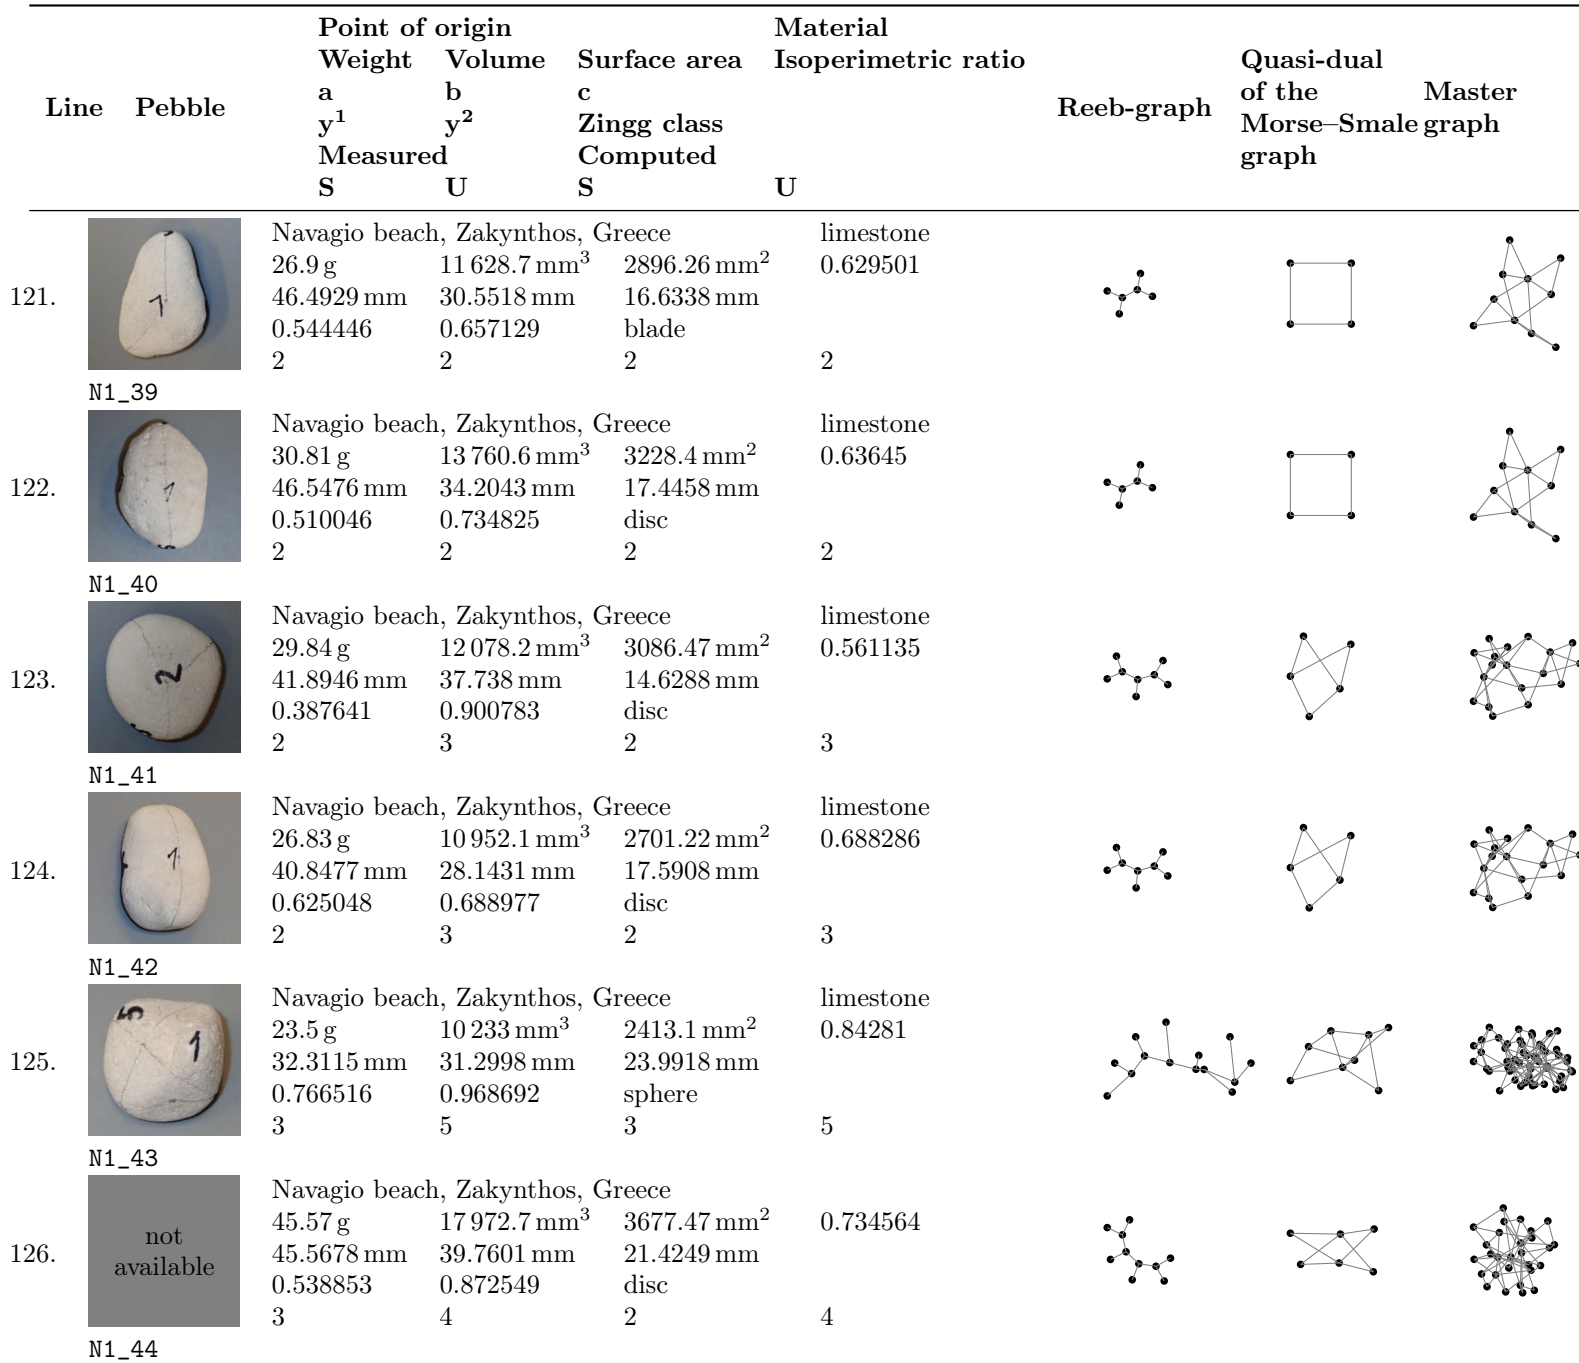 | 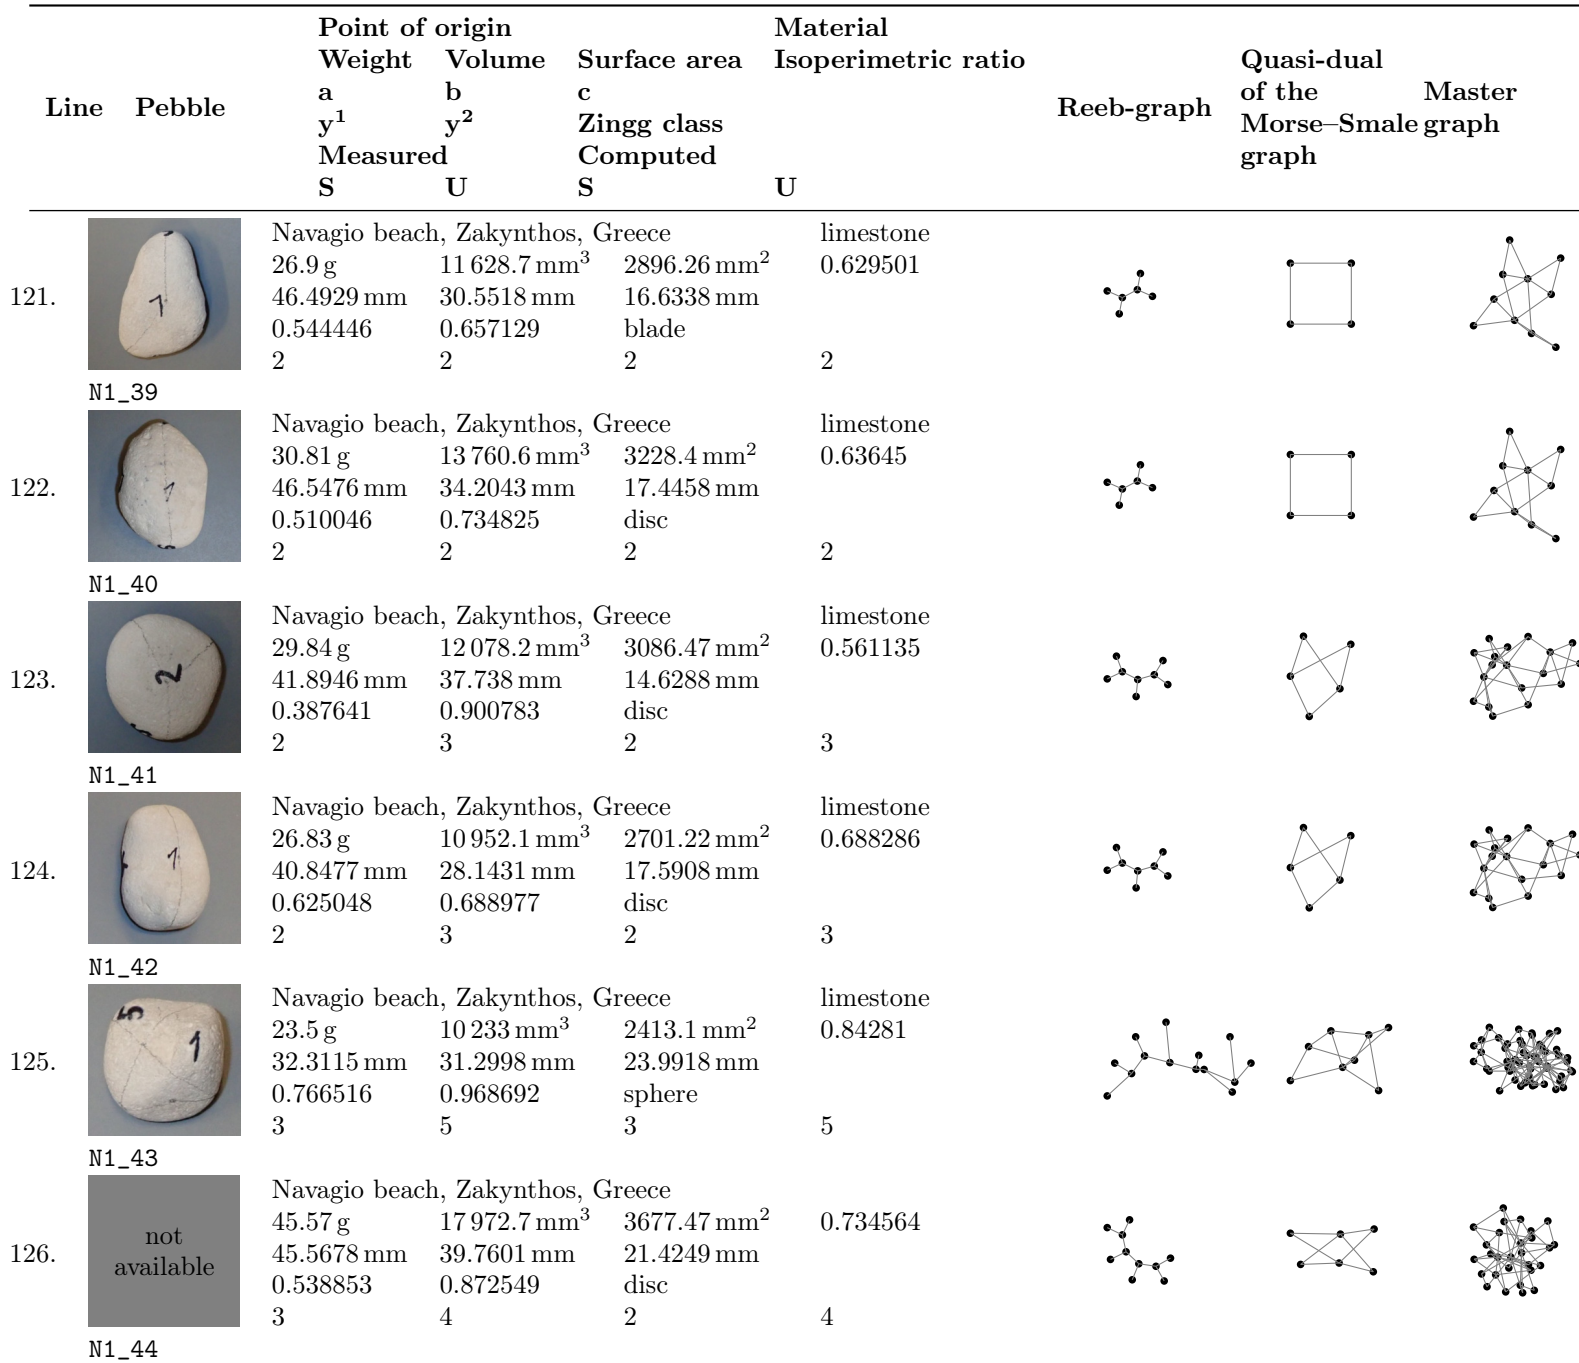 |
|      | N1_44                                                                               |                                                                            |                                                         |                                                     |                                |                                                                                       |                                                                                       |                                                                                       |

| Line  | Pebble                                                                              | Point of origin                                                            |                                                         |                                                      | Material                       |                                                                                       | Reeb-graph                                                                            | Quasi-dual<br>of the<br>Morse–Smale<br>graph                                          | Master<br>graph |
|-------|-------------------------------------------------------------------------------------|----------------------------------------------------------------------------|---------------------------------------------------------|------------------------------------------------------|--------------------------------|---------------------------------------------------------------------------------------|---------------------------------------------------------------------------------------|---------------------------------------------------------------------------------------|-----------------|
|       |                                                                                     | Weight                                                                     | Volume                                                  | Surface area                                         | Isoperimetric ratio            |                                                                                       |                                                                                       |                                                                                       |                 |
|       |                                                                                     | a                                                                          | b                                                       | c                                                    |                                |                                                                                       |                                                                                       |                                                                                       |                 |
|       |                                                                                     | y <sup>1</sup><br>Measured<br>S                                            | y <sup>2</sup><br>U                                     | Zingg class<br>Computed<br>S                         | U                              |                                                                                       |                                                                                       |                                                                                       |                 |
| 127.  | 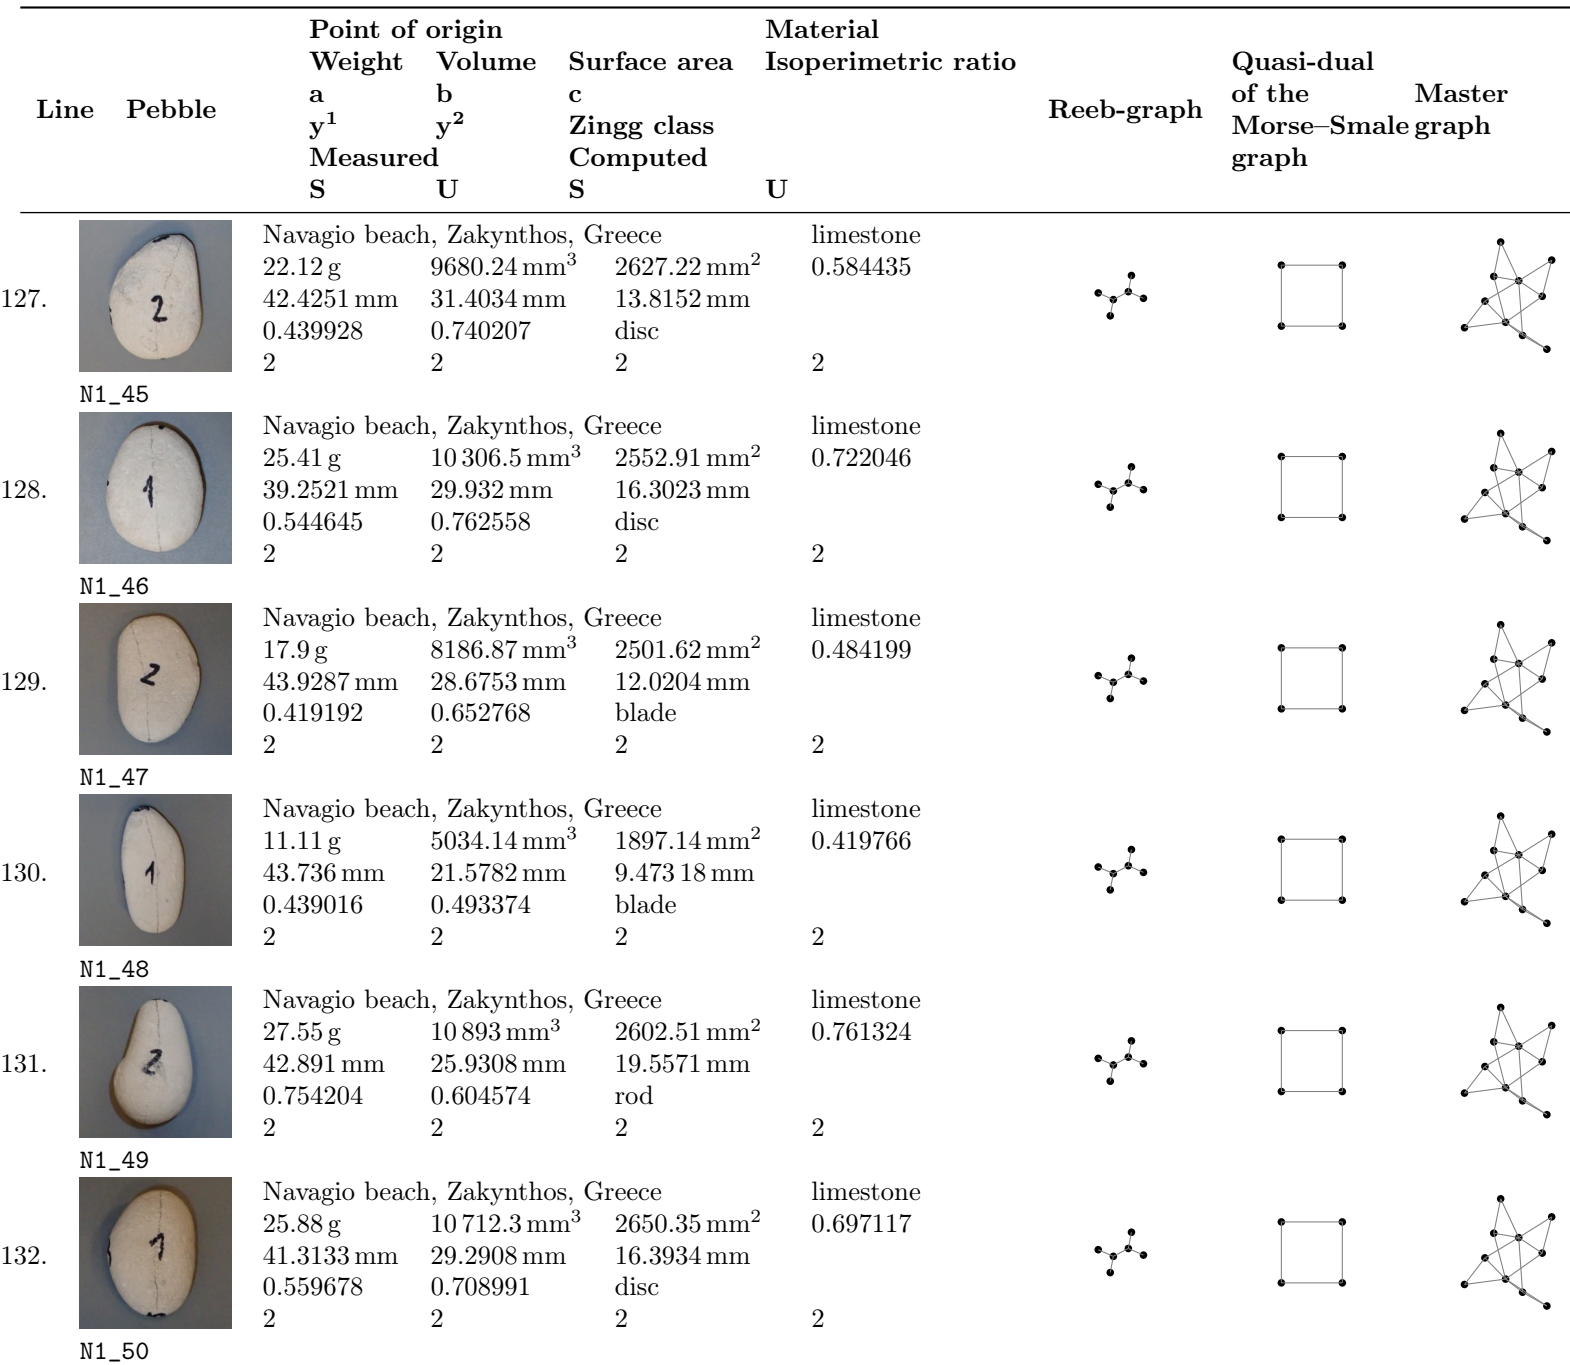   | Navagio beach, Zakynthos, Greece<br>22.12 g<br>42.4251 mm<br>0.439928<br>2 | 9680.24 mm <sup>3</sup><br>31.4034 mm<br>0.740207<br>2  | 2627.22 mm <sup>2</sup><br>13.8152 mm<br>disc<br>2   | limestone<br>0.584435<br><br>2 | 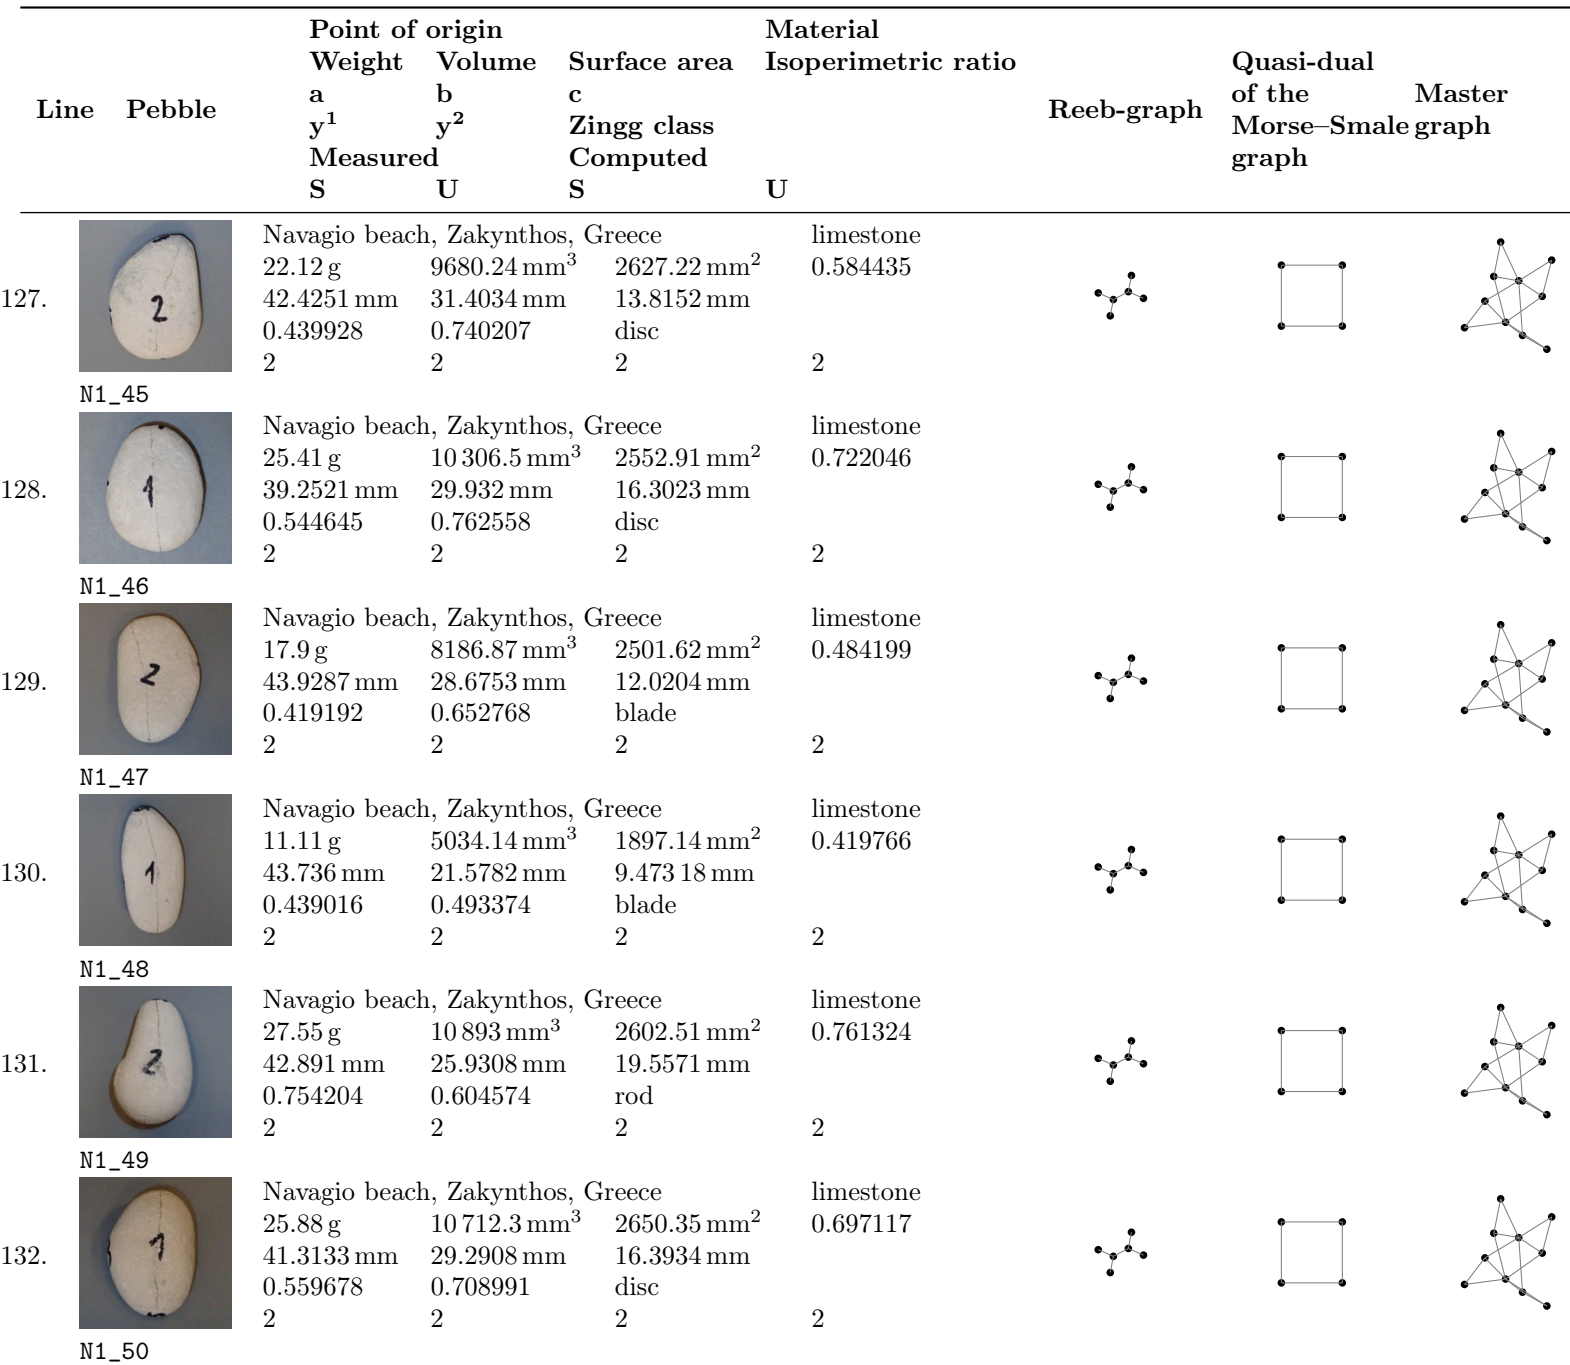   | 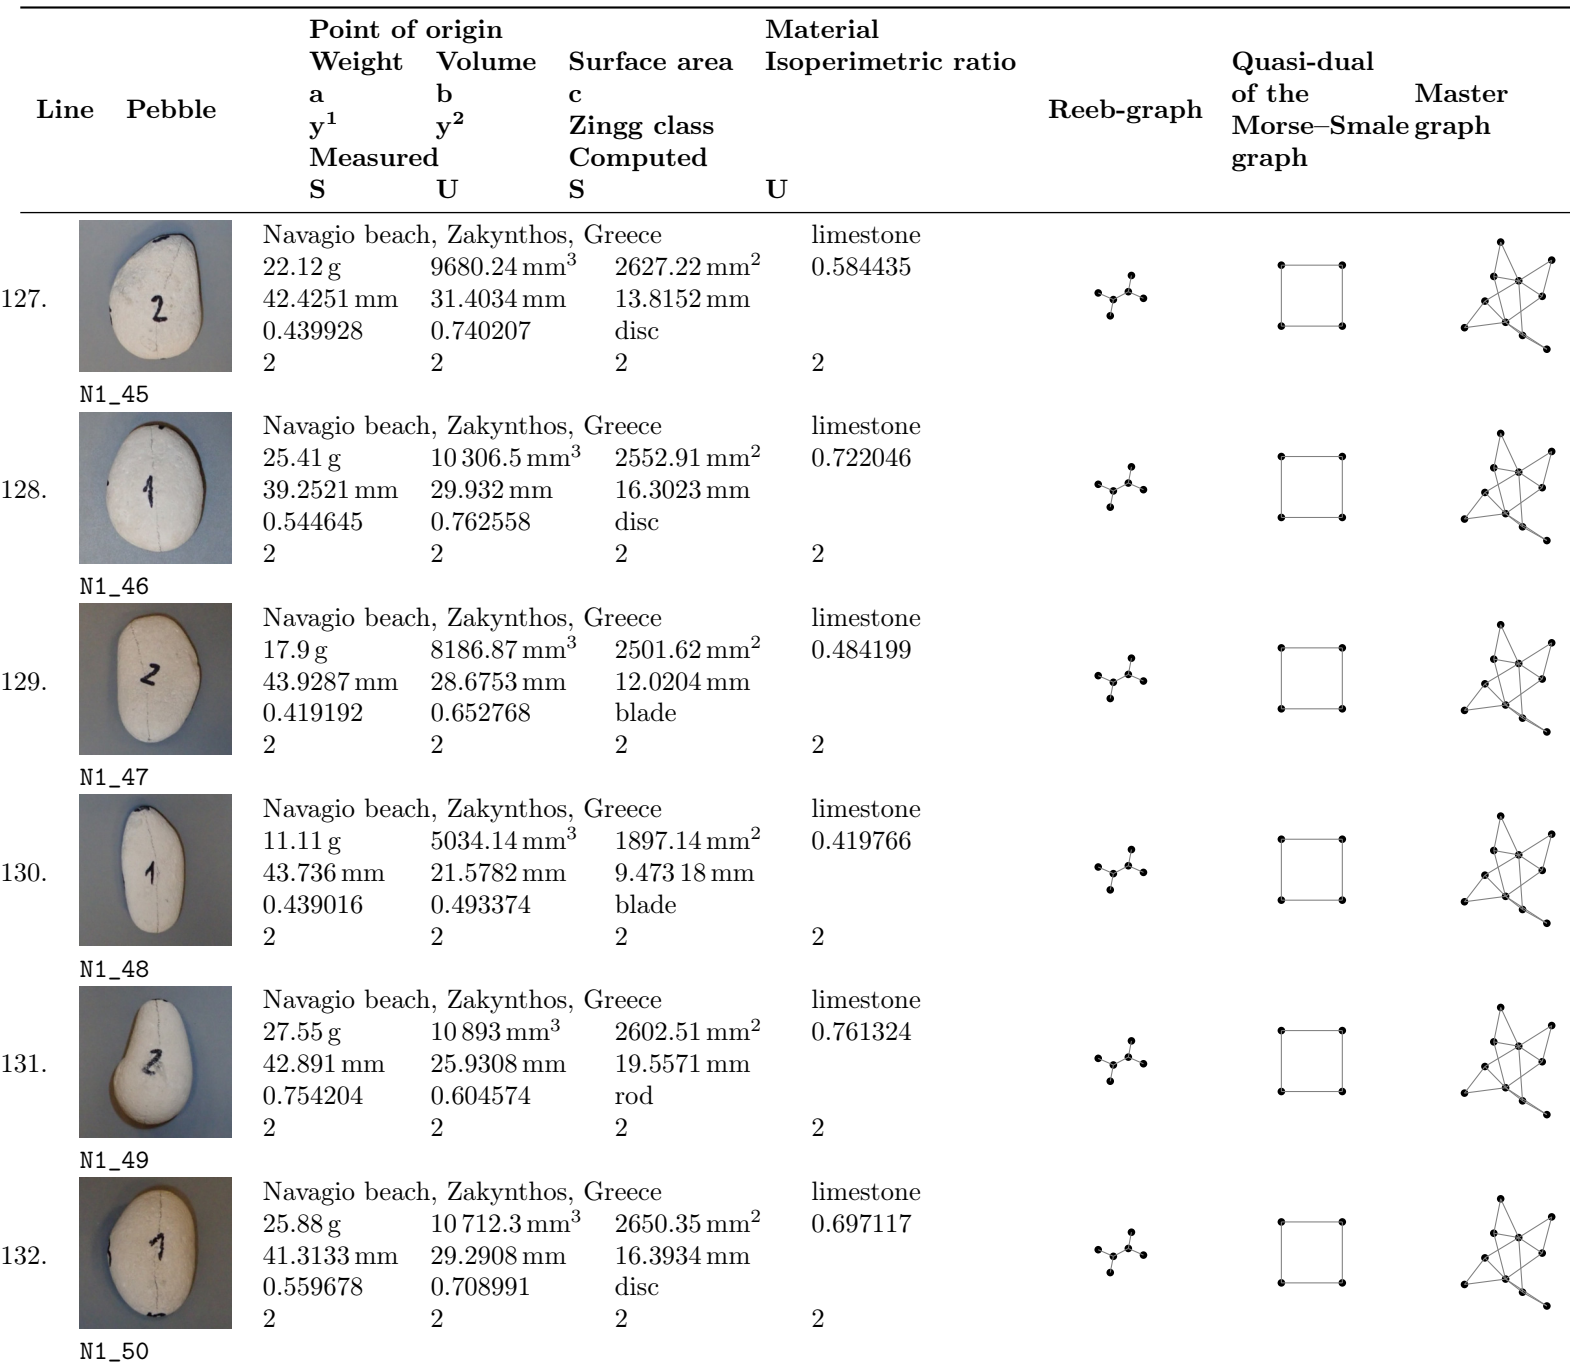   | 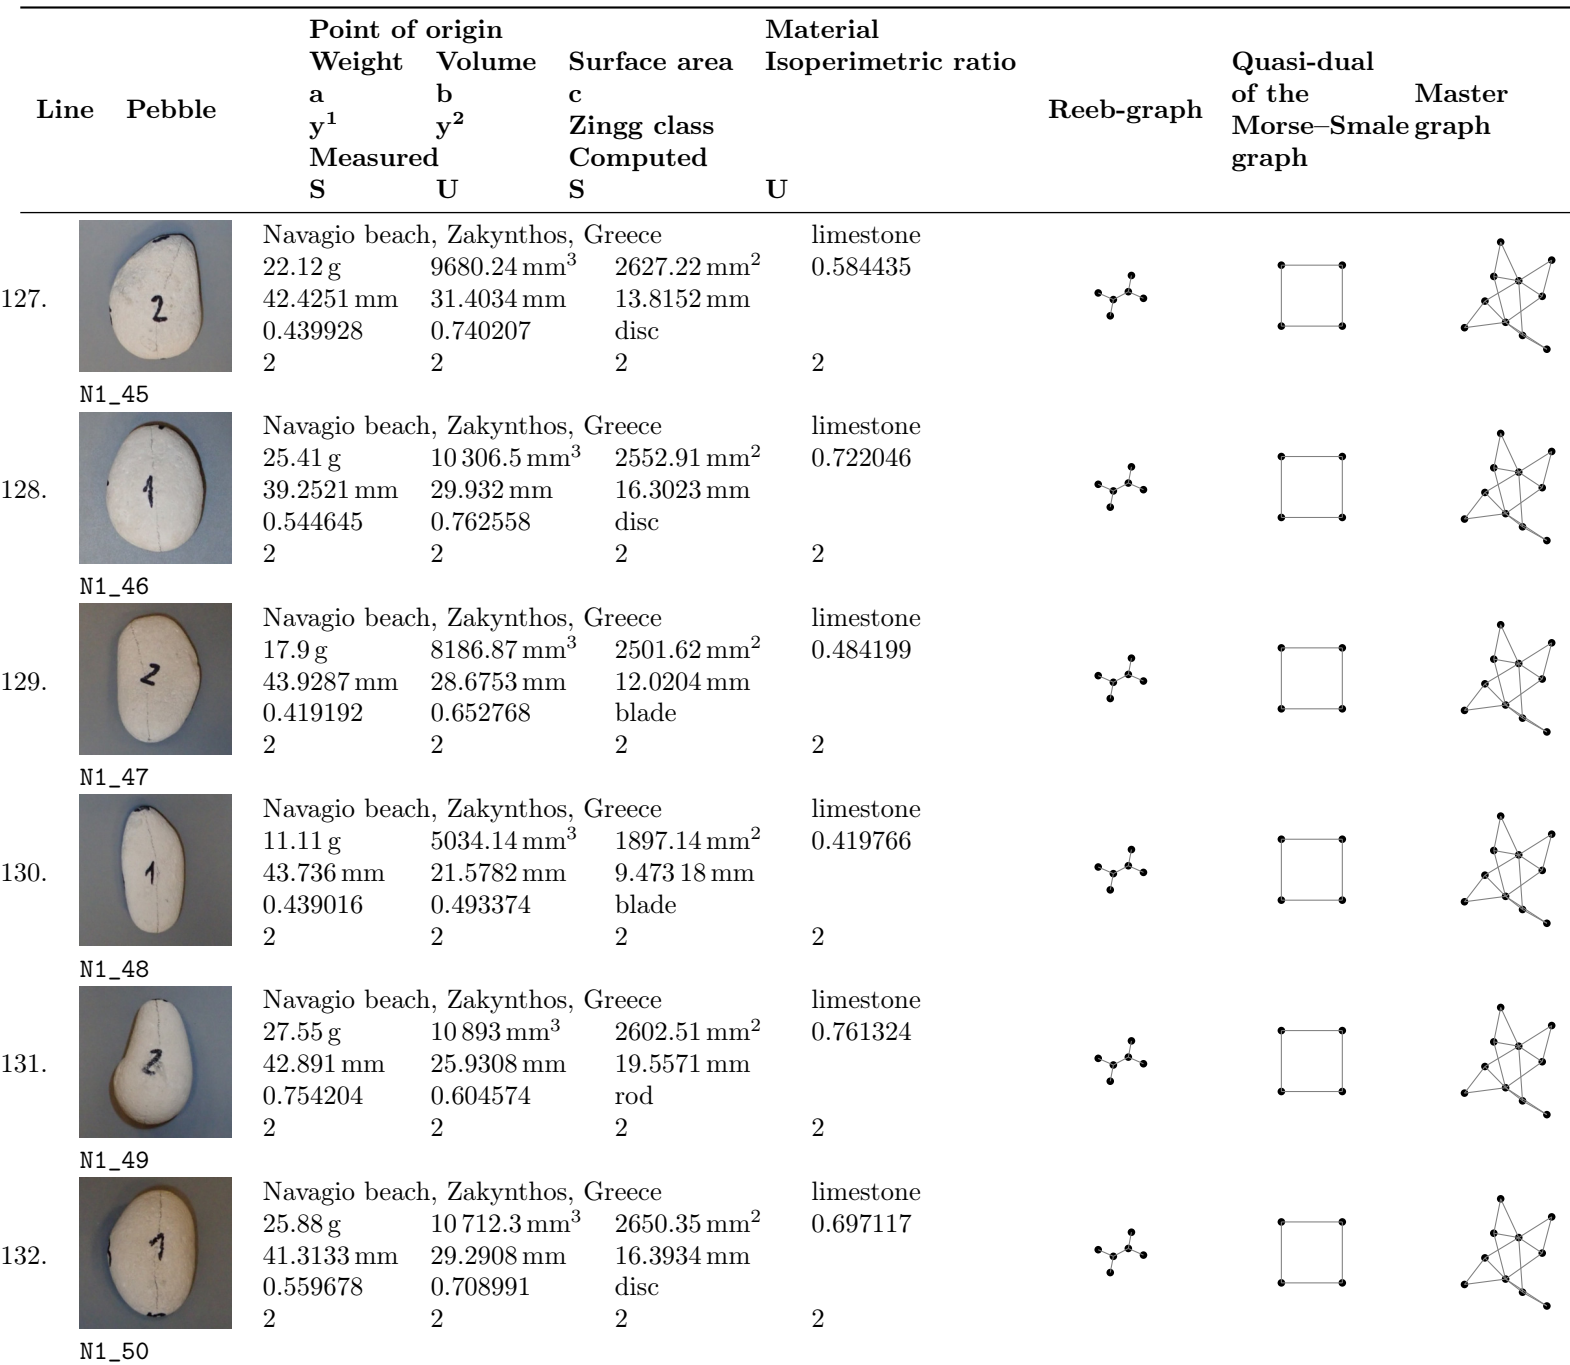   |                 |
| N1_45 |                                                                                     |                                                                            |                                                         |                                                      |                                |                                                                                       |                                                                                       |                                                                                       |                 |
| 128.  | 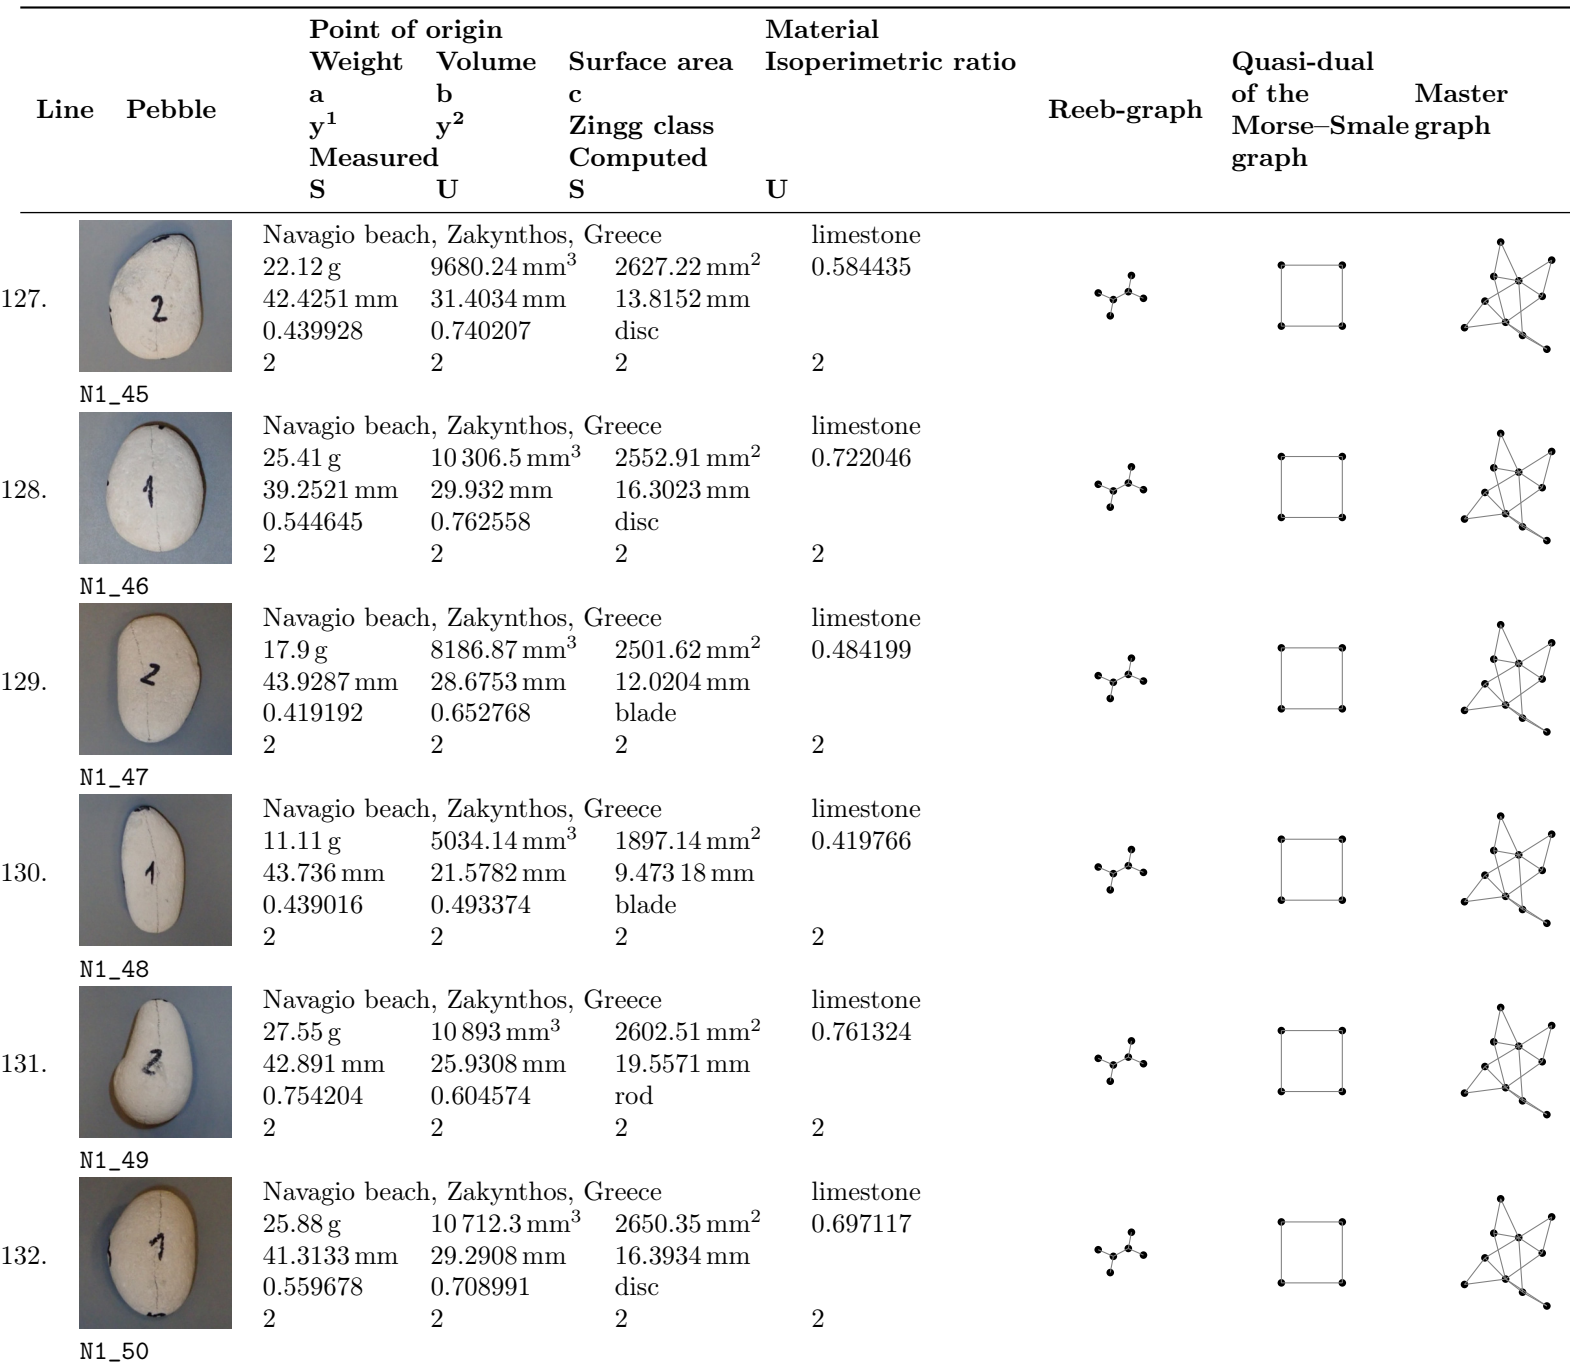   | Navagio beach, Zakynthos, Greece<br>25.41 g<br>39.2521 mm<br>0.544645<br>2 | 10 306.5 mm <sup>3</sup><br>29.932 mm<br>0.762558<br>2  | 2552.91 mm <sup>2</sup><br>16.3023 mm<br>disc<br>2   | limestone<br>0.722046<br><br>2 | 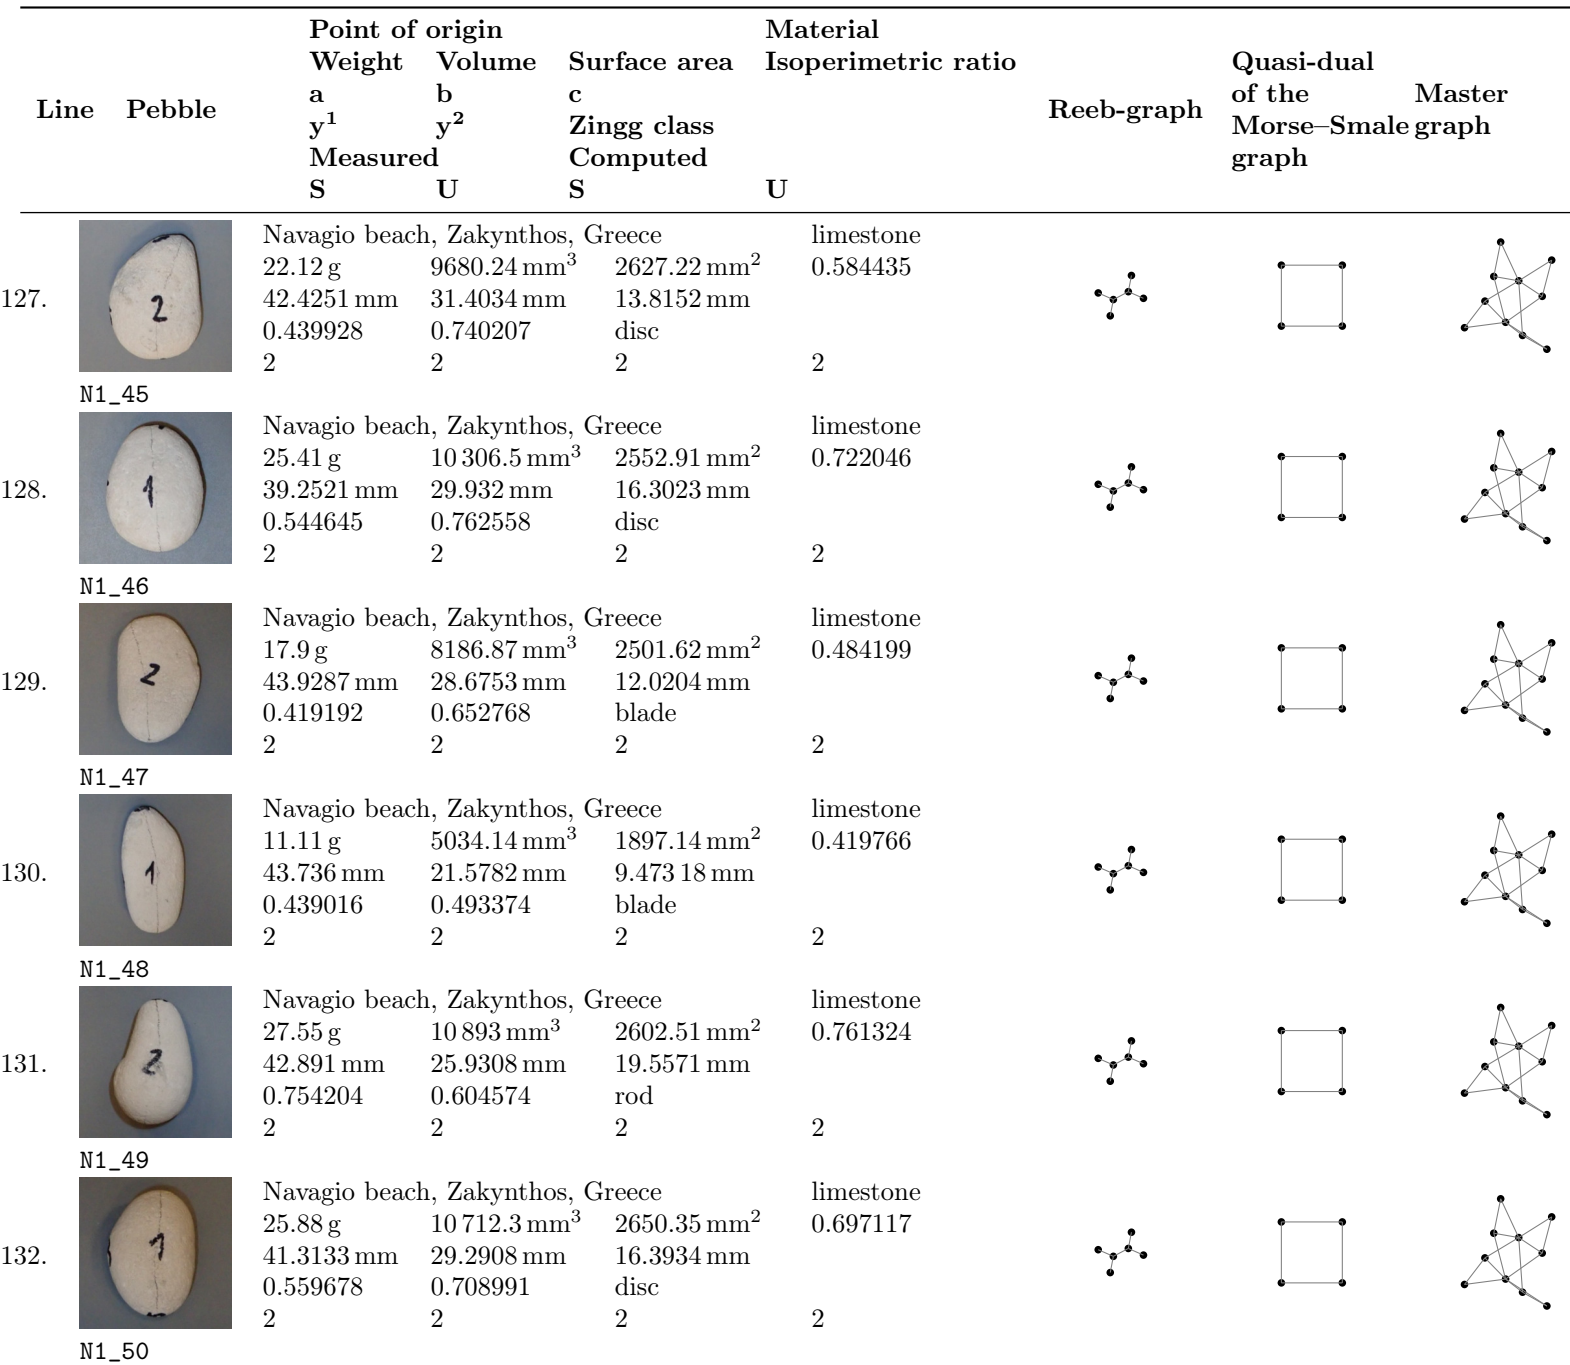   | 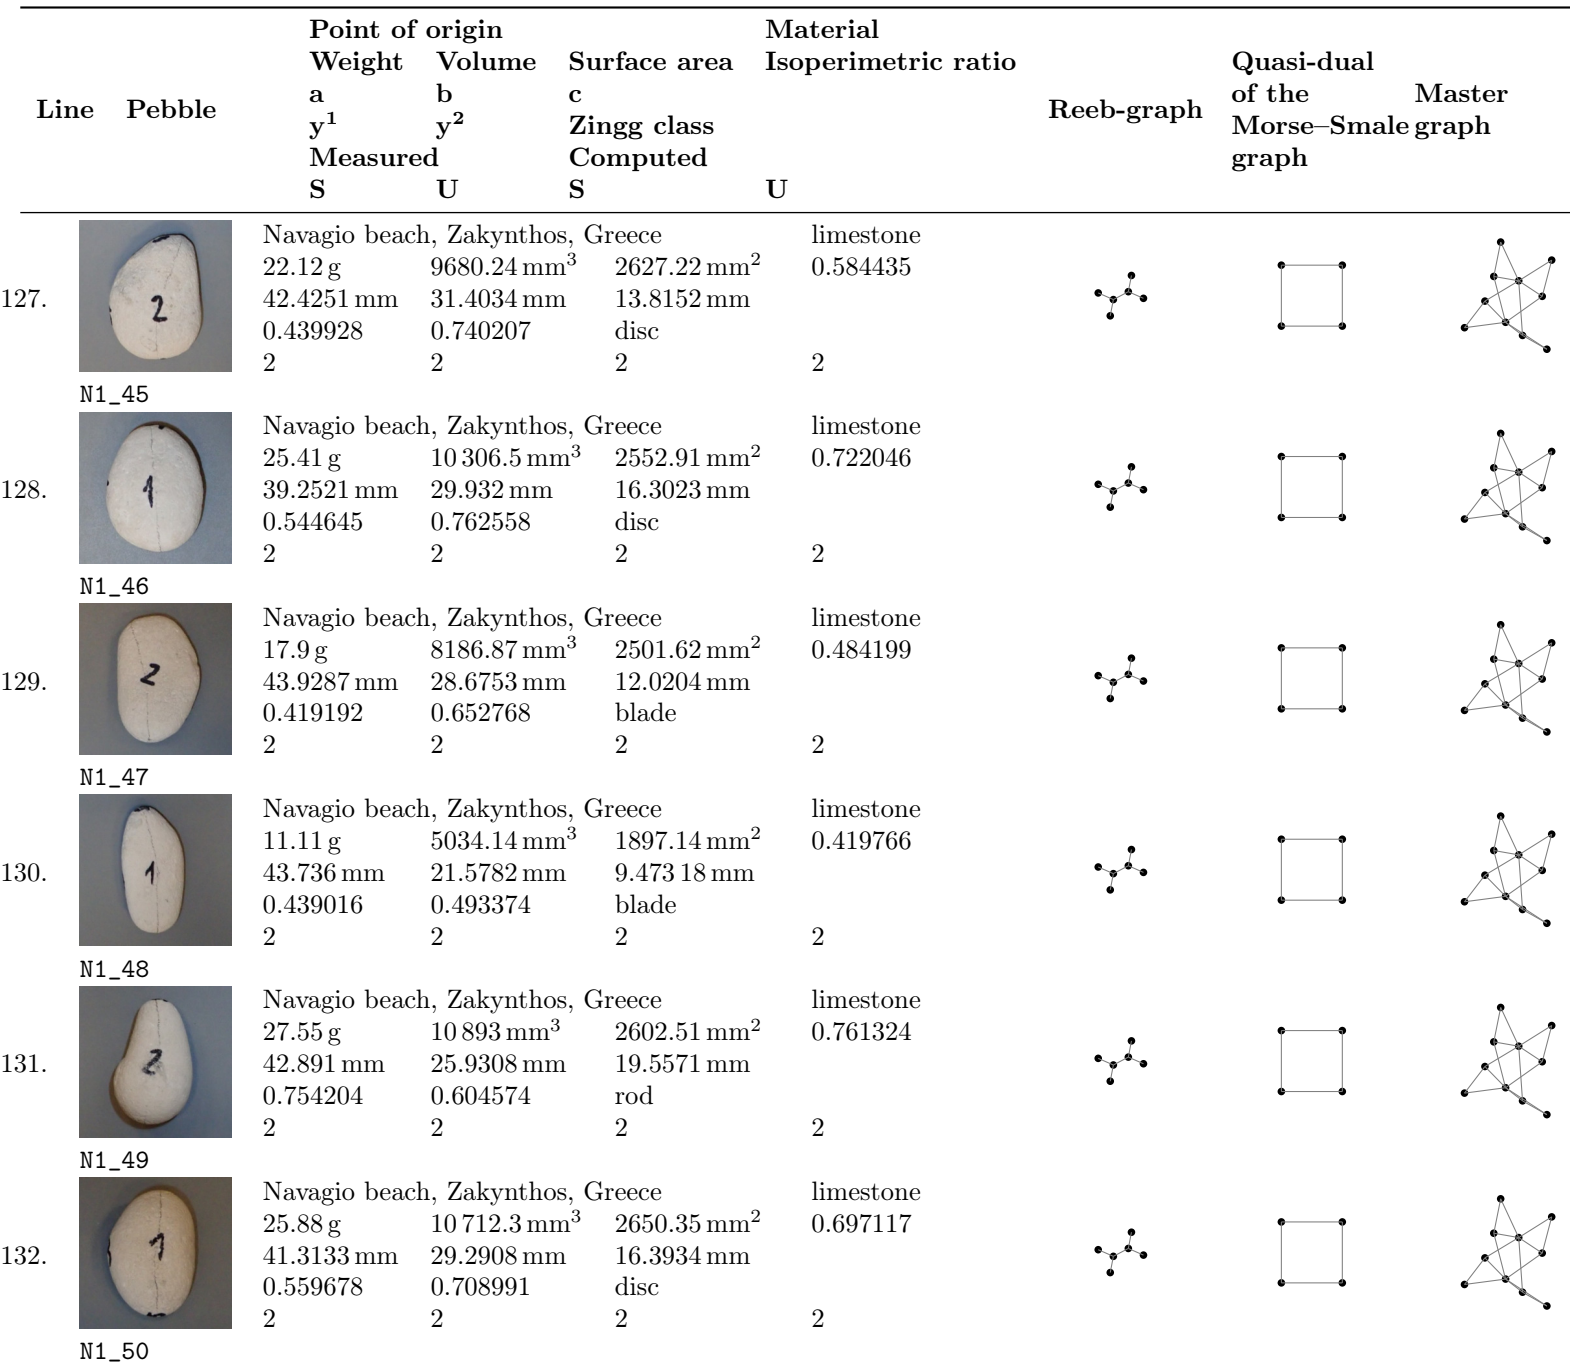   | 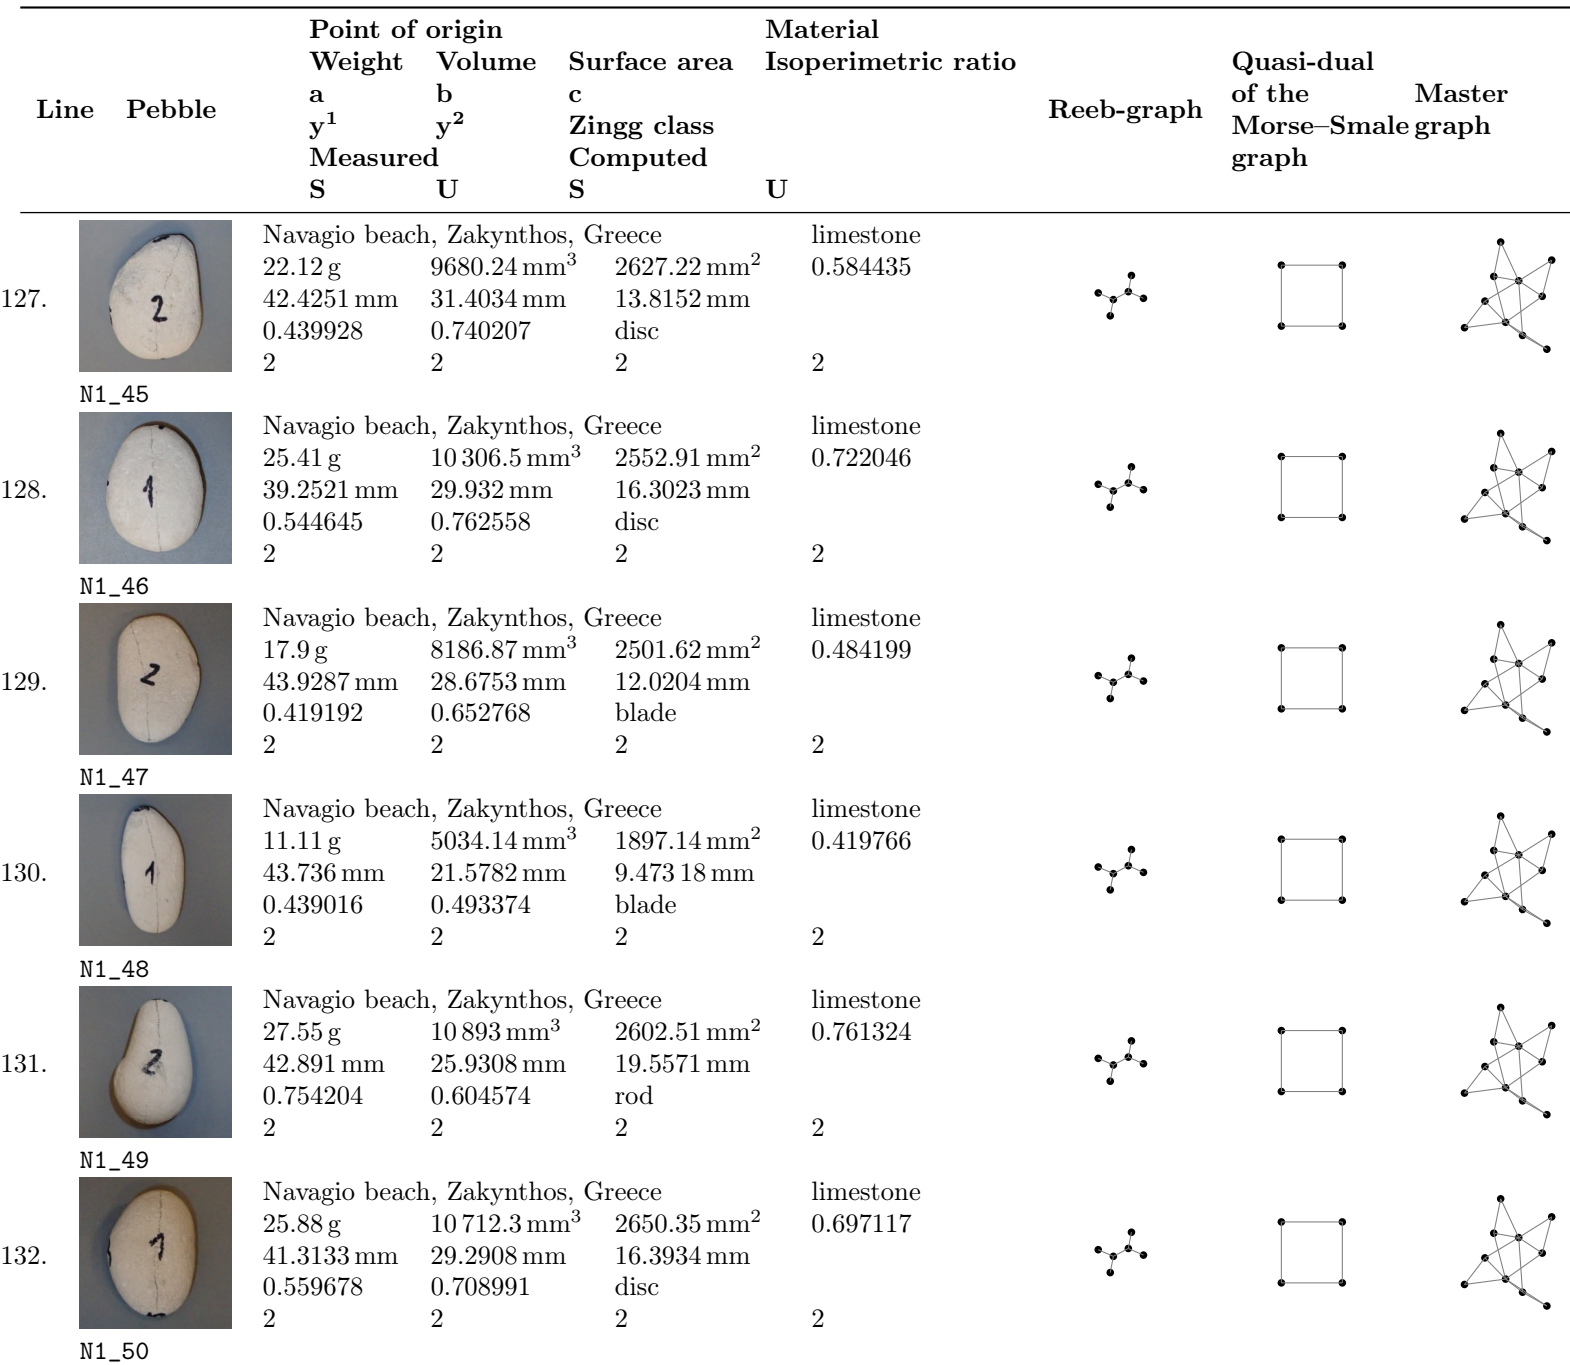   |                 |
| N1_46 |                                                                                     |                                                                            |                                                         |                                                      |                                |                                                                                       |                                                                                       |                                                                                       |                 |
| 129.  | 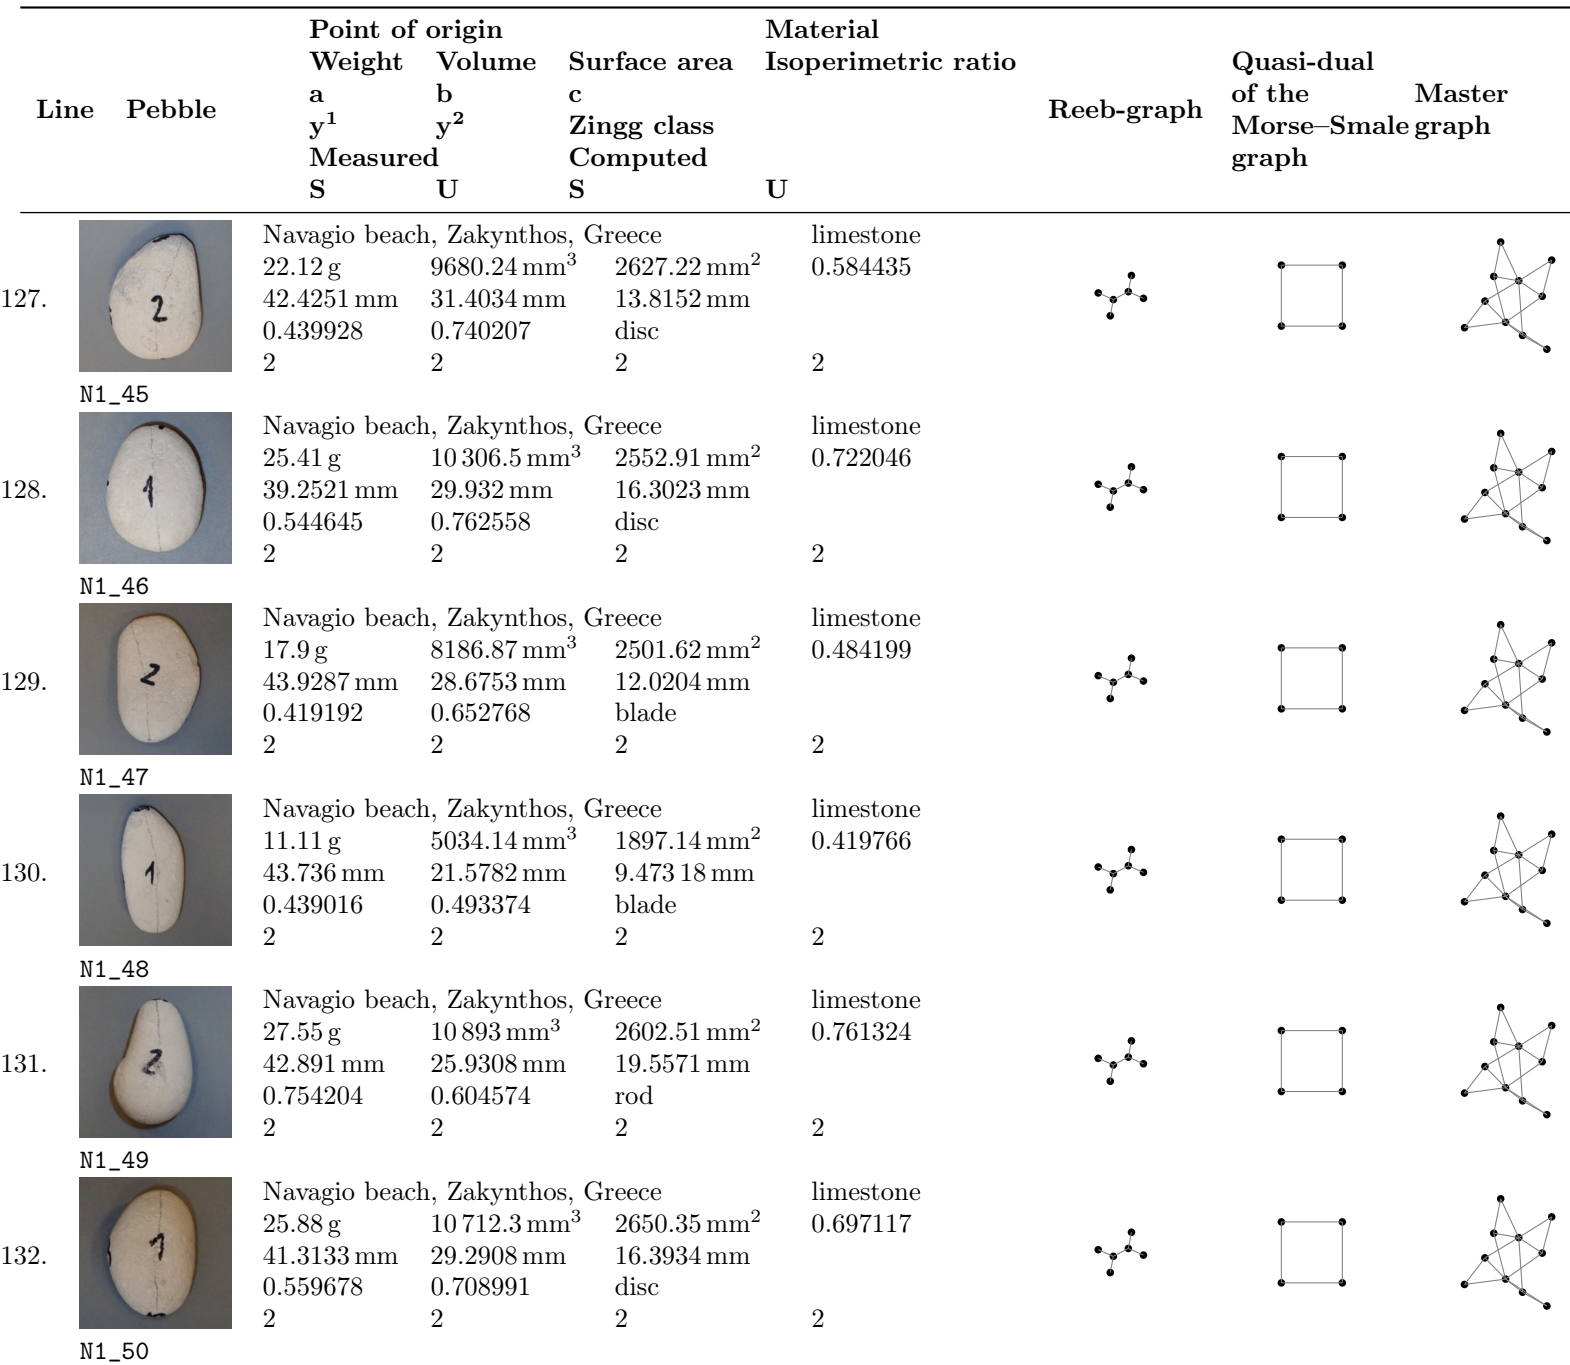   | Navagio beach, Zakynthos, Greece<br>17.9 g<br>43.9287 mm<br>0.419192<br>2  | 8186.87 mm <sup>3</sup><br>28.6753 mm<br>0.652768<br>2  | 2501.62 mm <sup>2</sup><br>12.0204 mm<br>blade<br>2  | limestone<br>0.484199<br><br>2 | 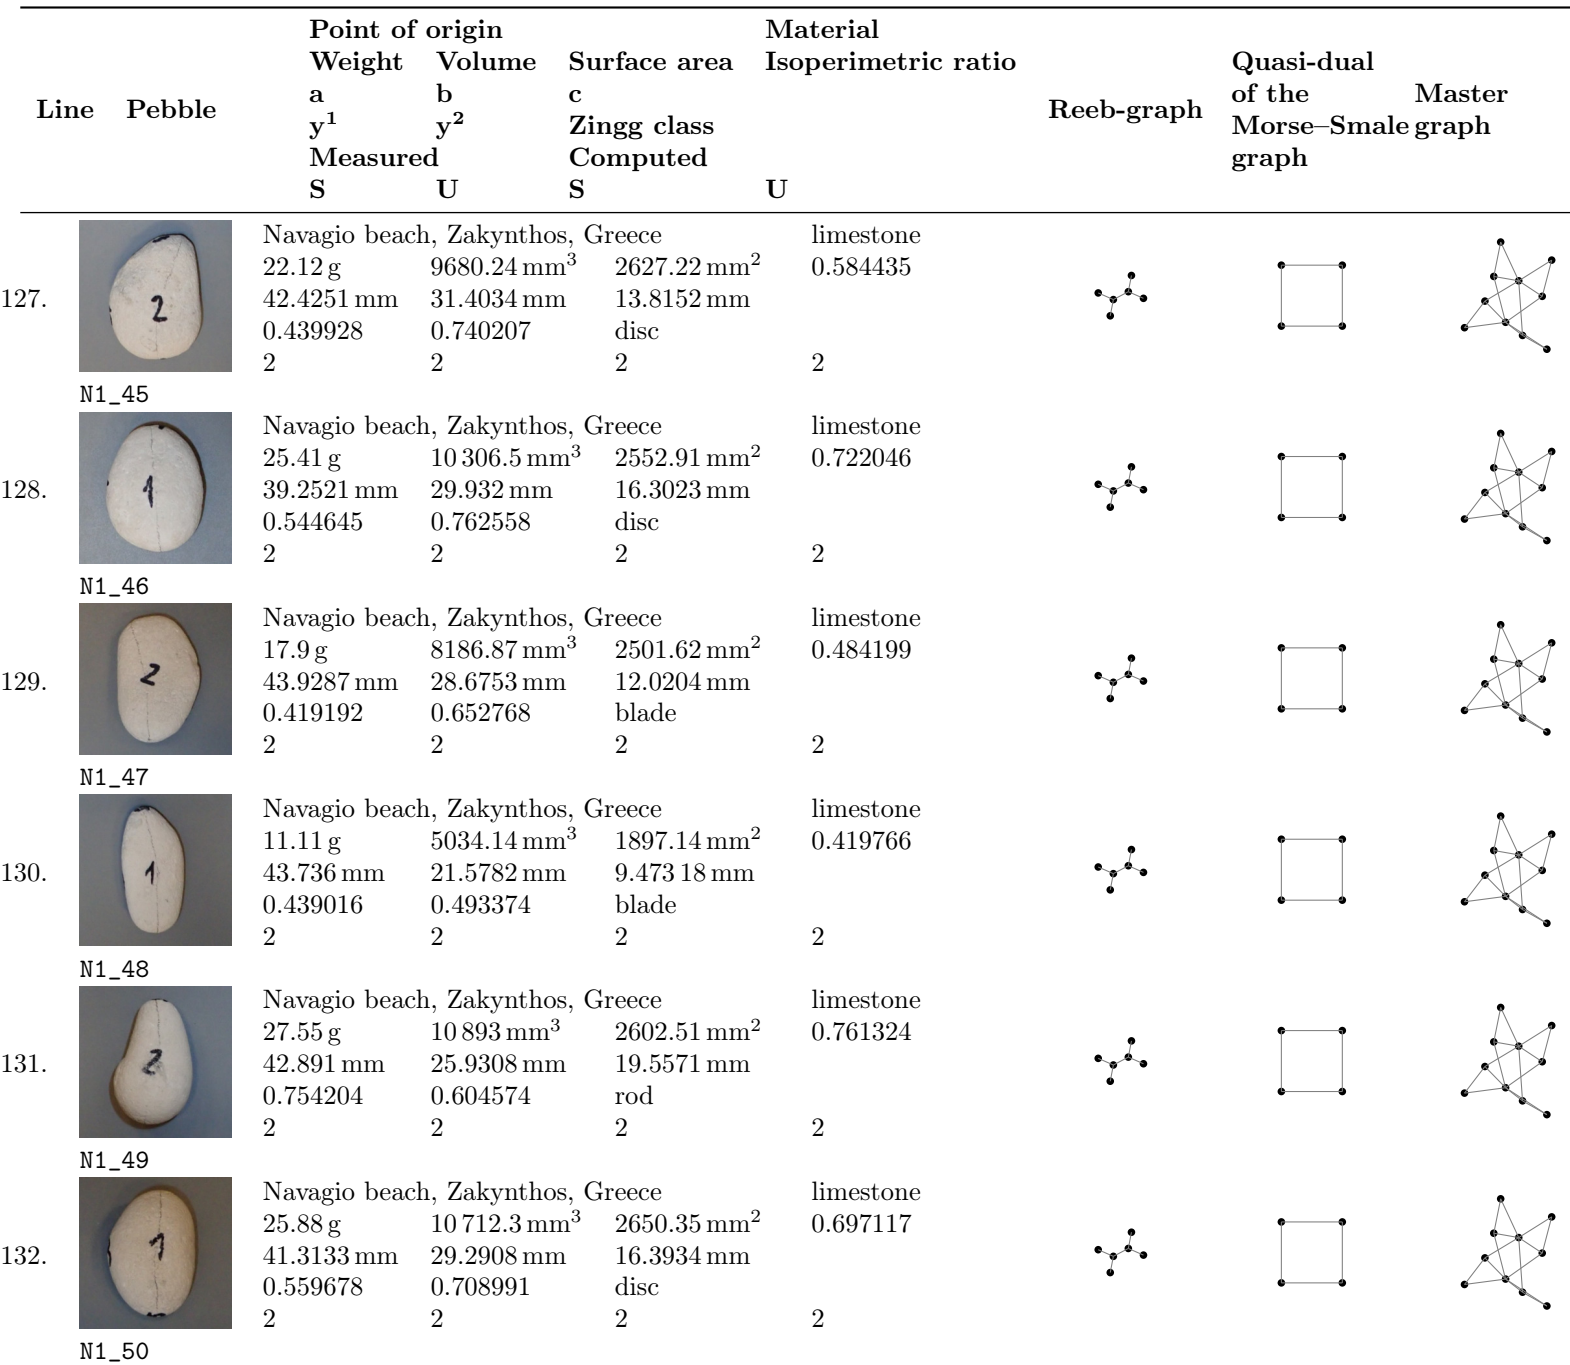   | 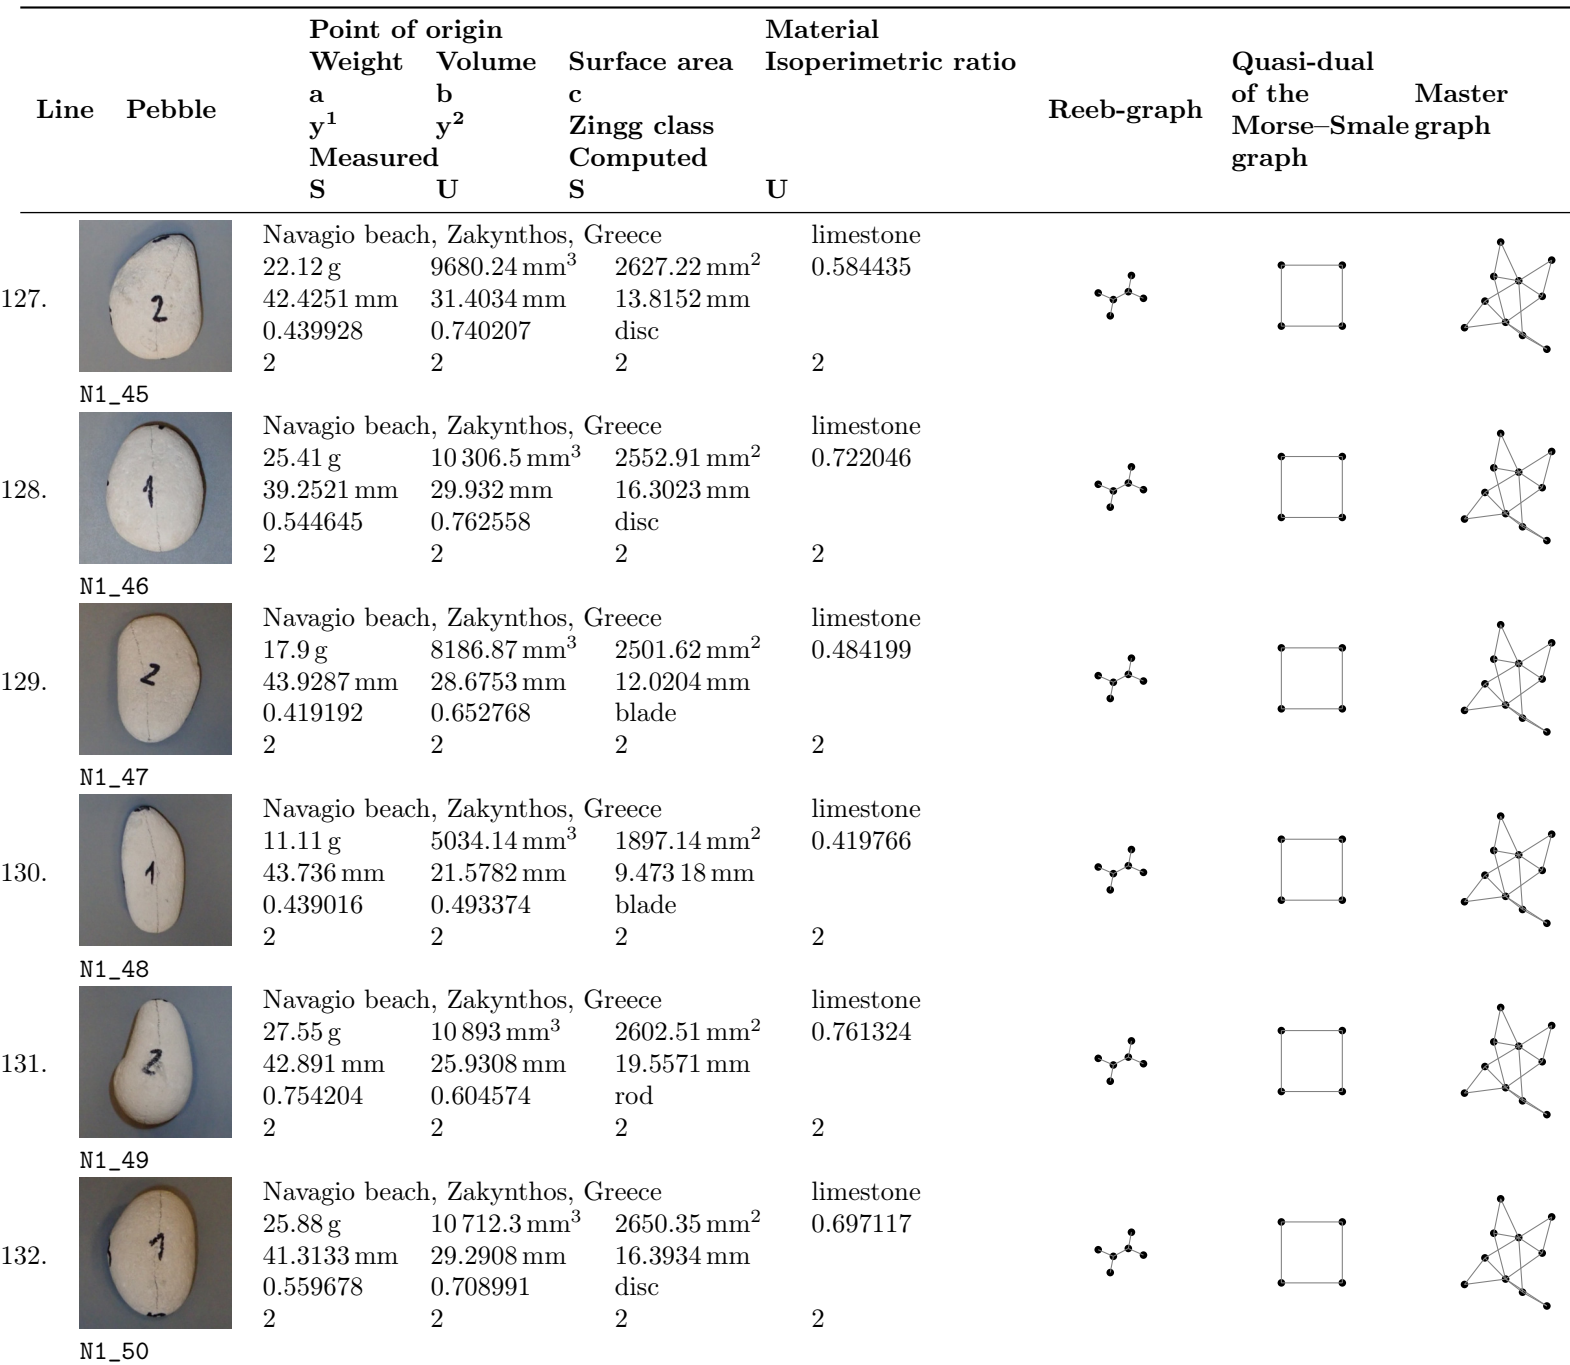   | 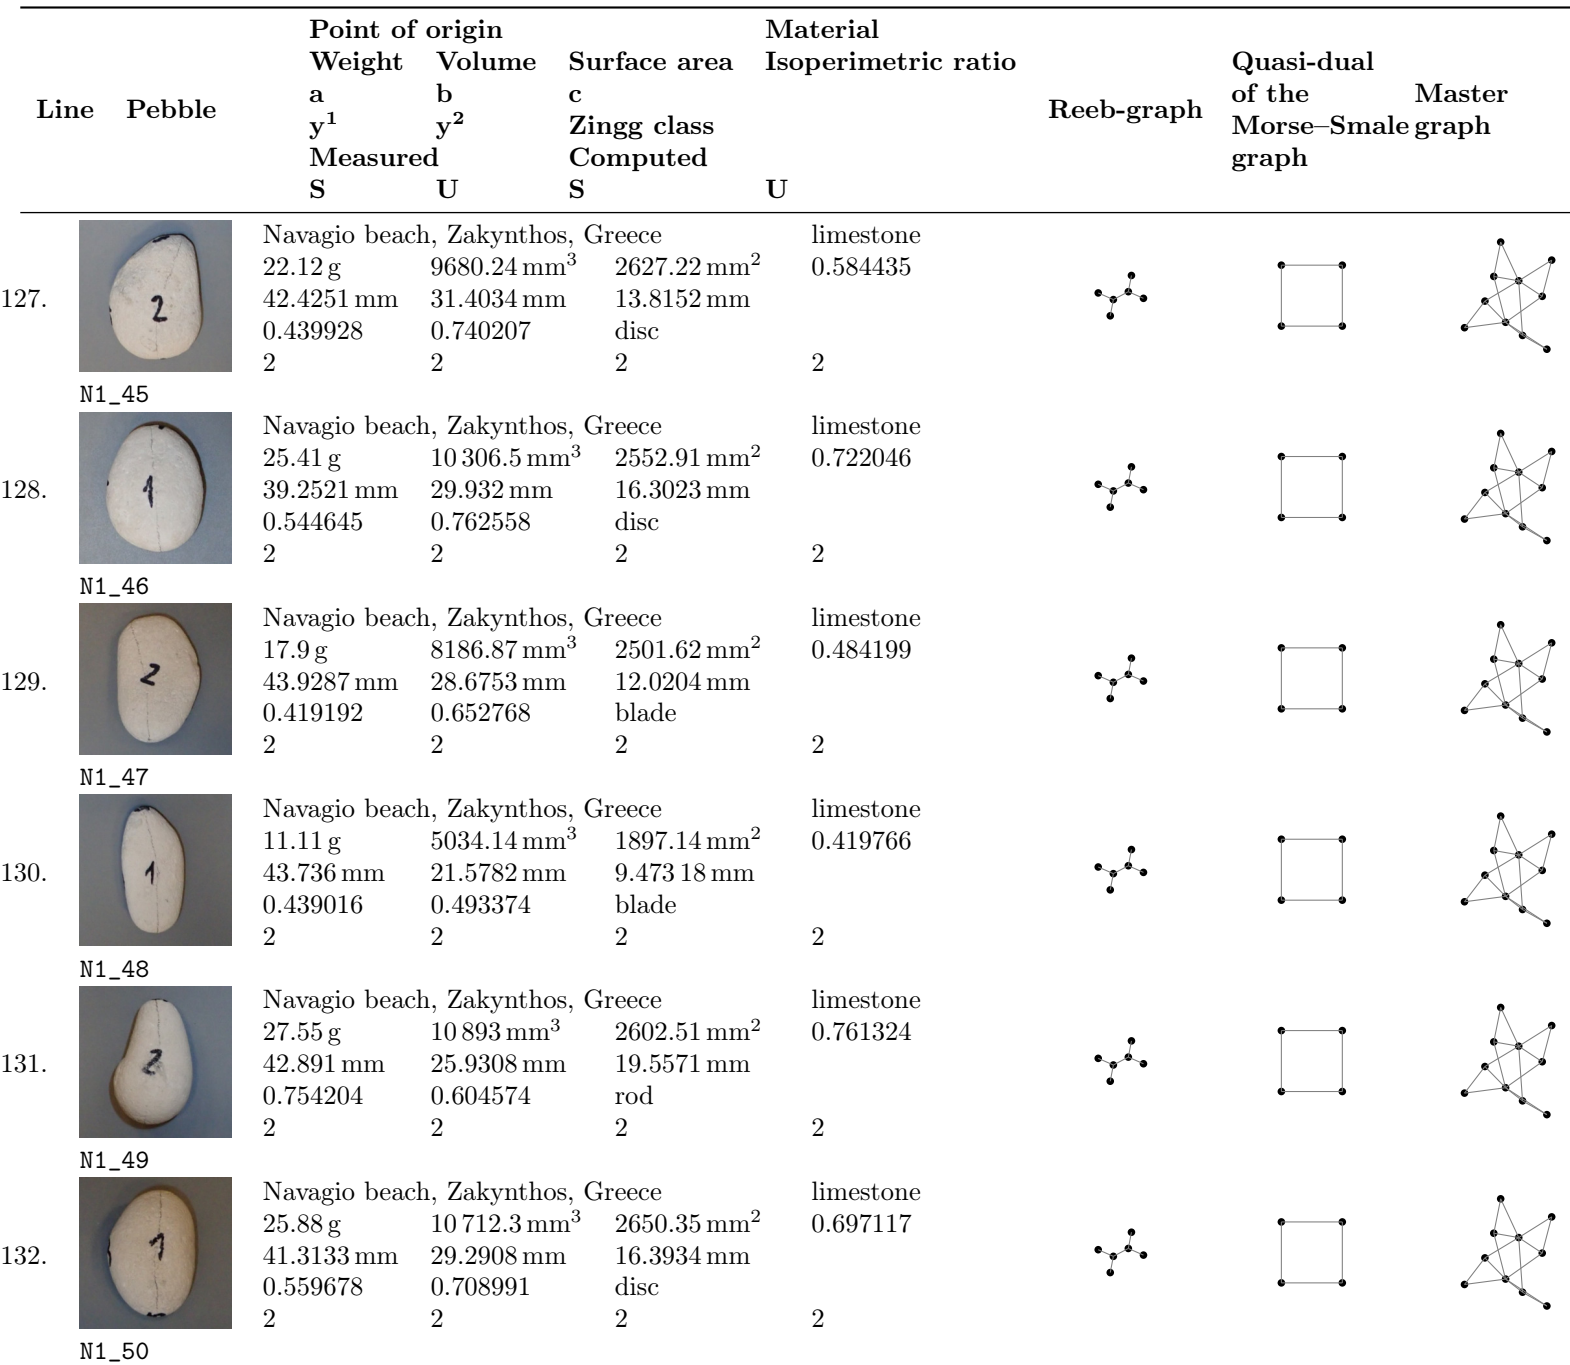   |                 |
| N1_47 |                                                                                     |                                                                            |                                                         |                                                      |                                |                                                                                       |                                                                                       |                                                                                       |                 |
| 130.  | 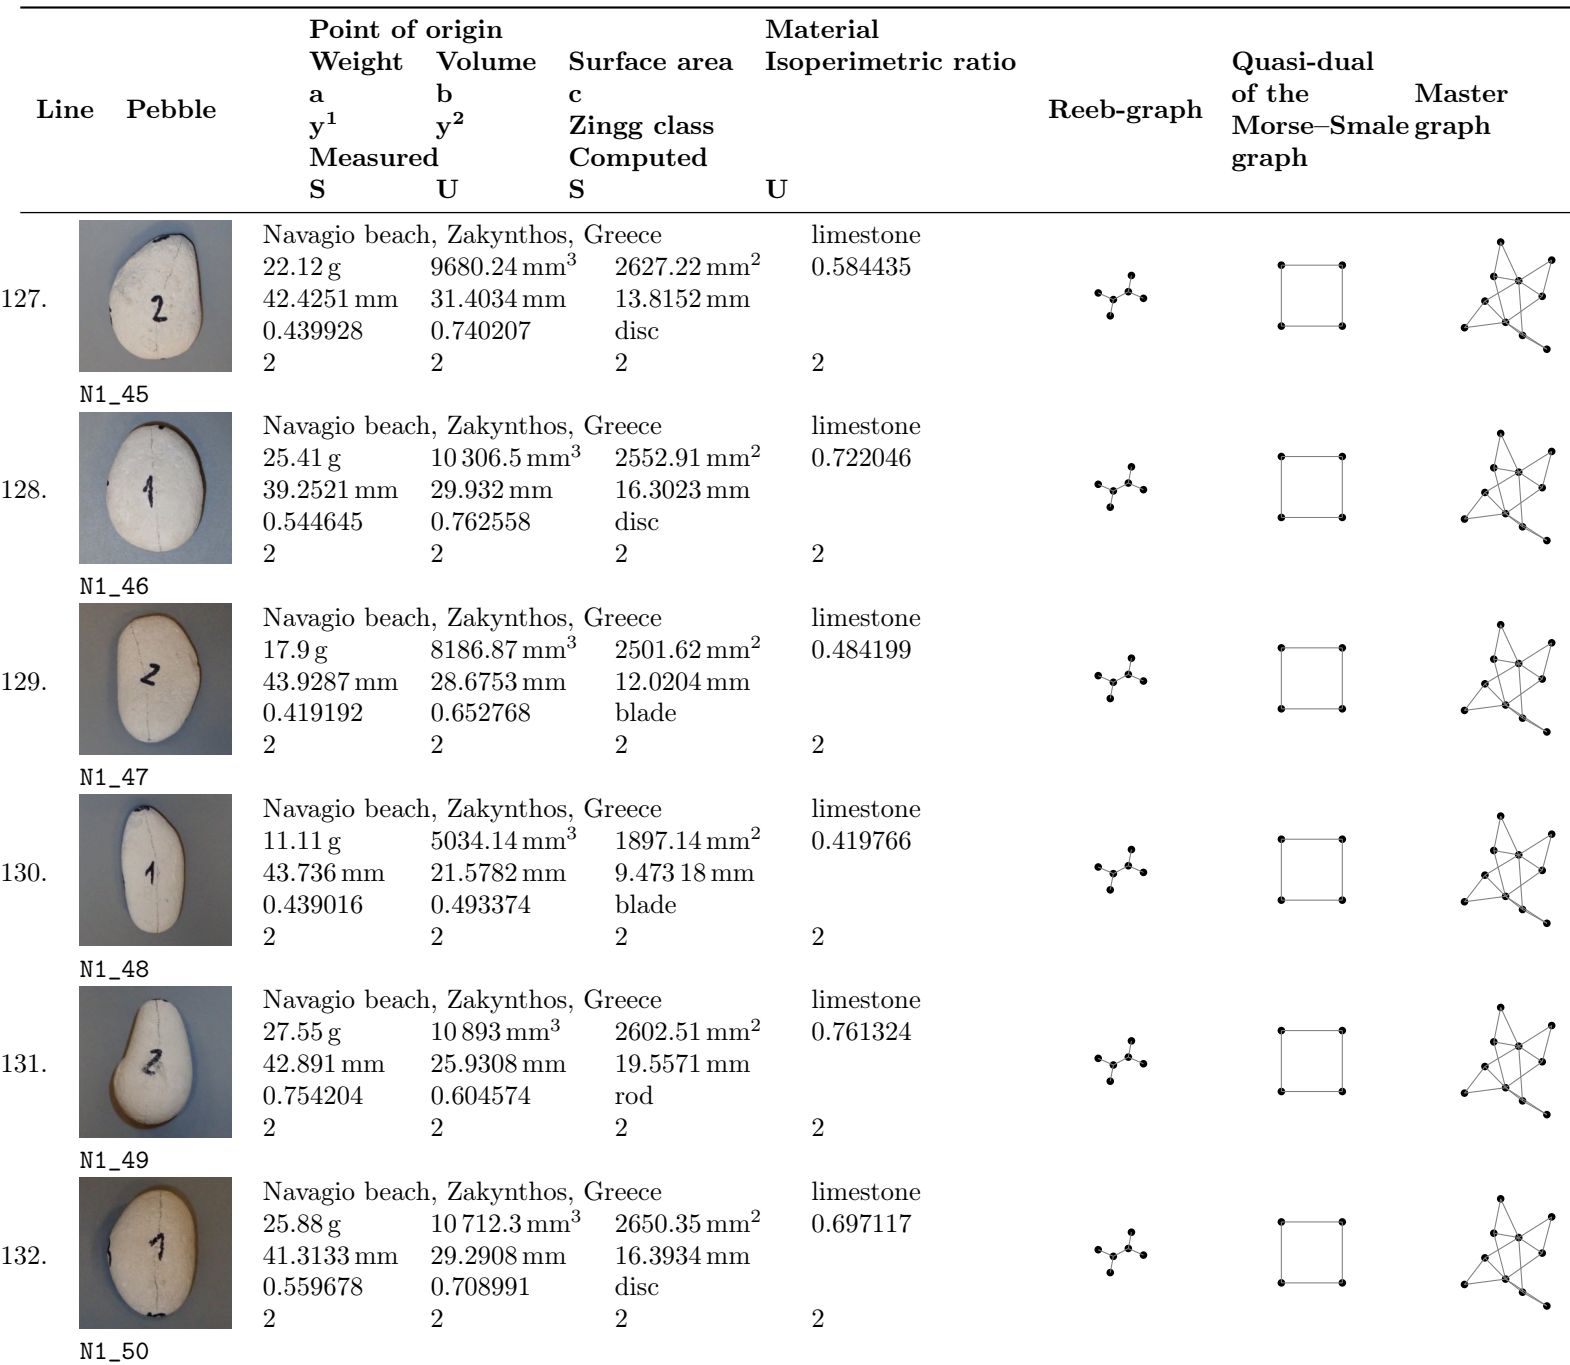  | Navagio beach, Zakynthos, Greece<br>11.11 g<br>43.736 mm<br>0.439016<br>2  | 5034.14 mm <sup>3</sup><br>21.5782 mm<br>0.493374<br>2  | 1897.14 mm <sup>2</sup><br>9.473 18 mm<br>blade<br>2 | limestone<br>0.419766<br><br>2 | 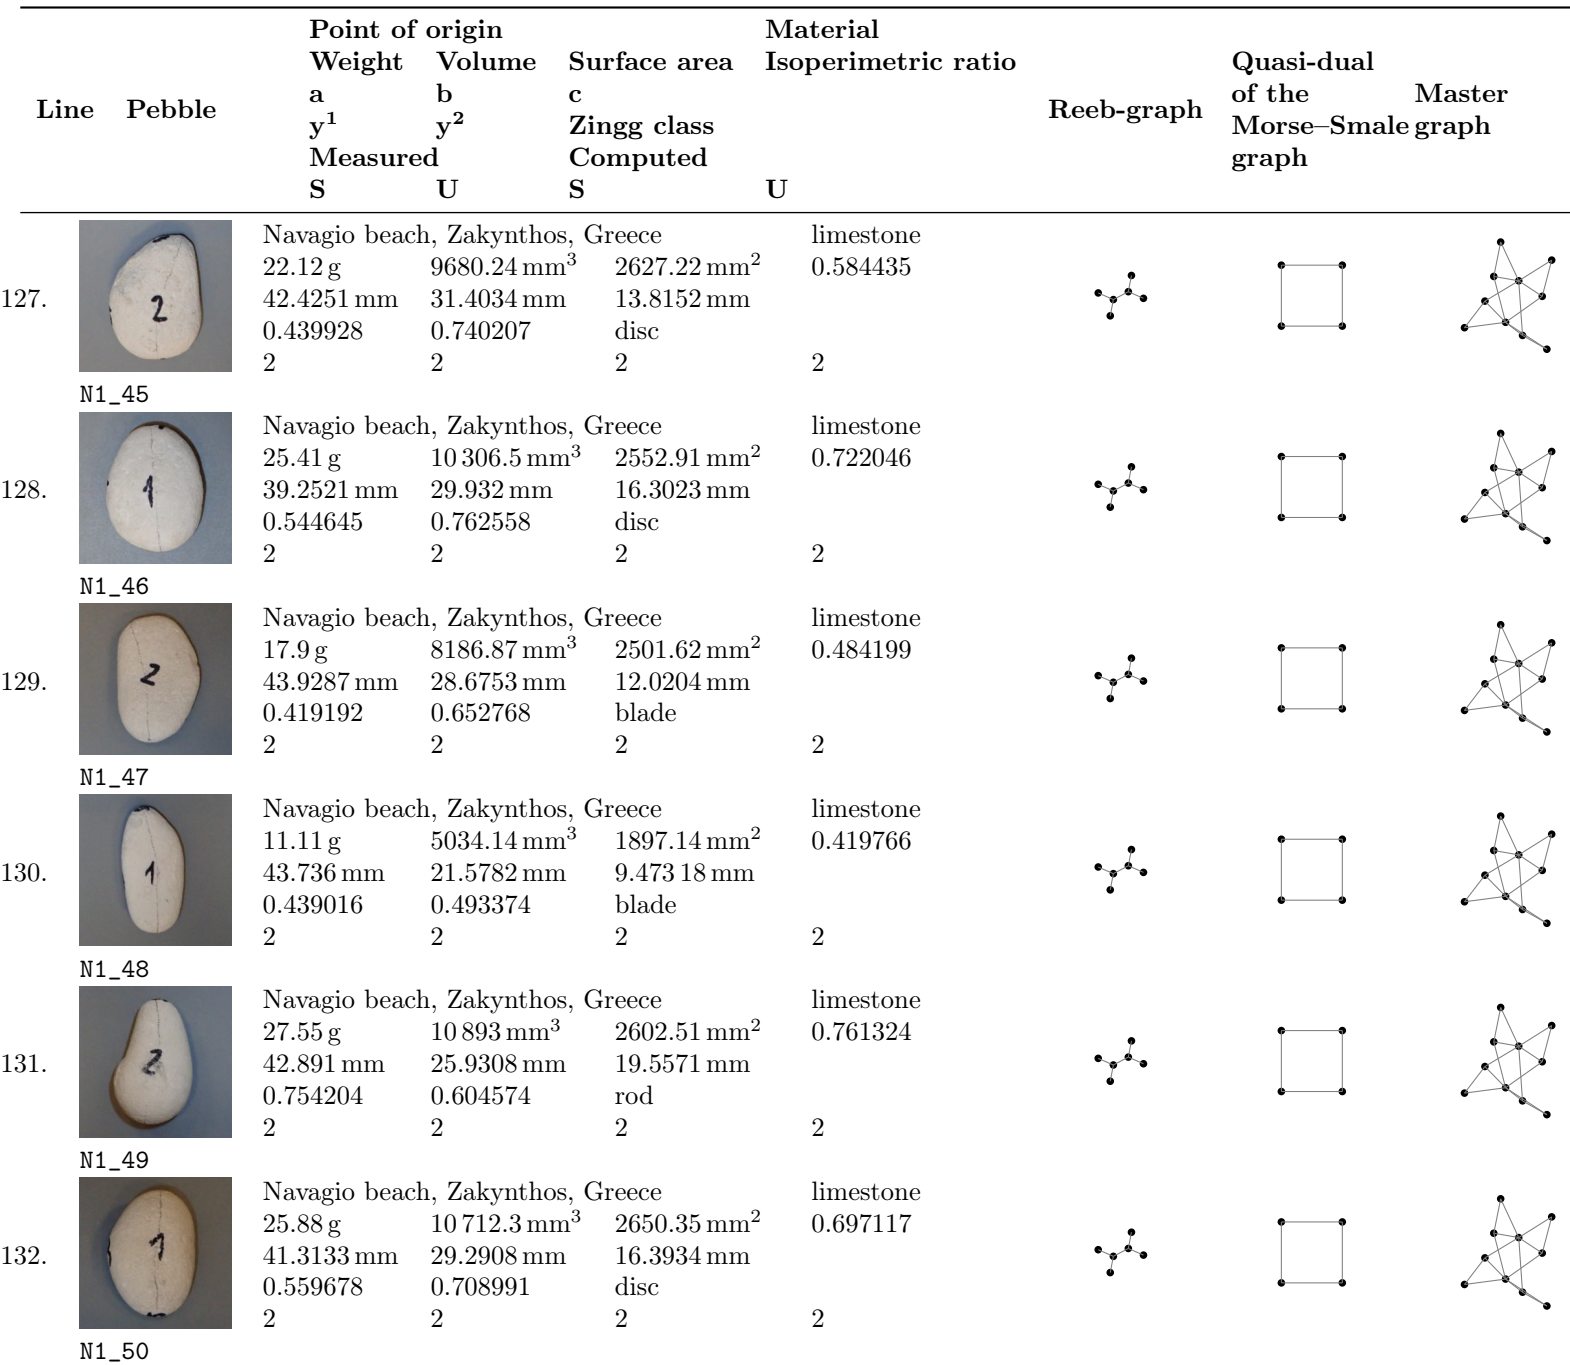  | 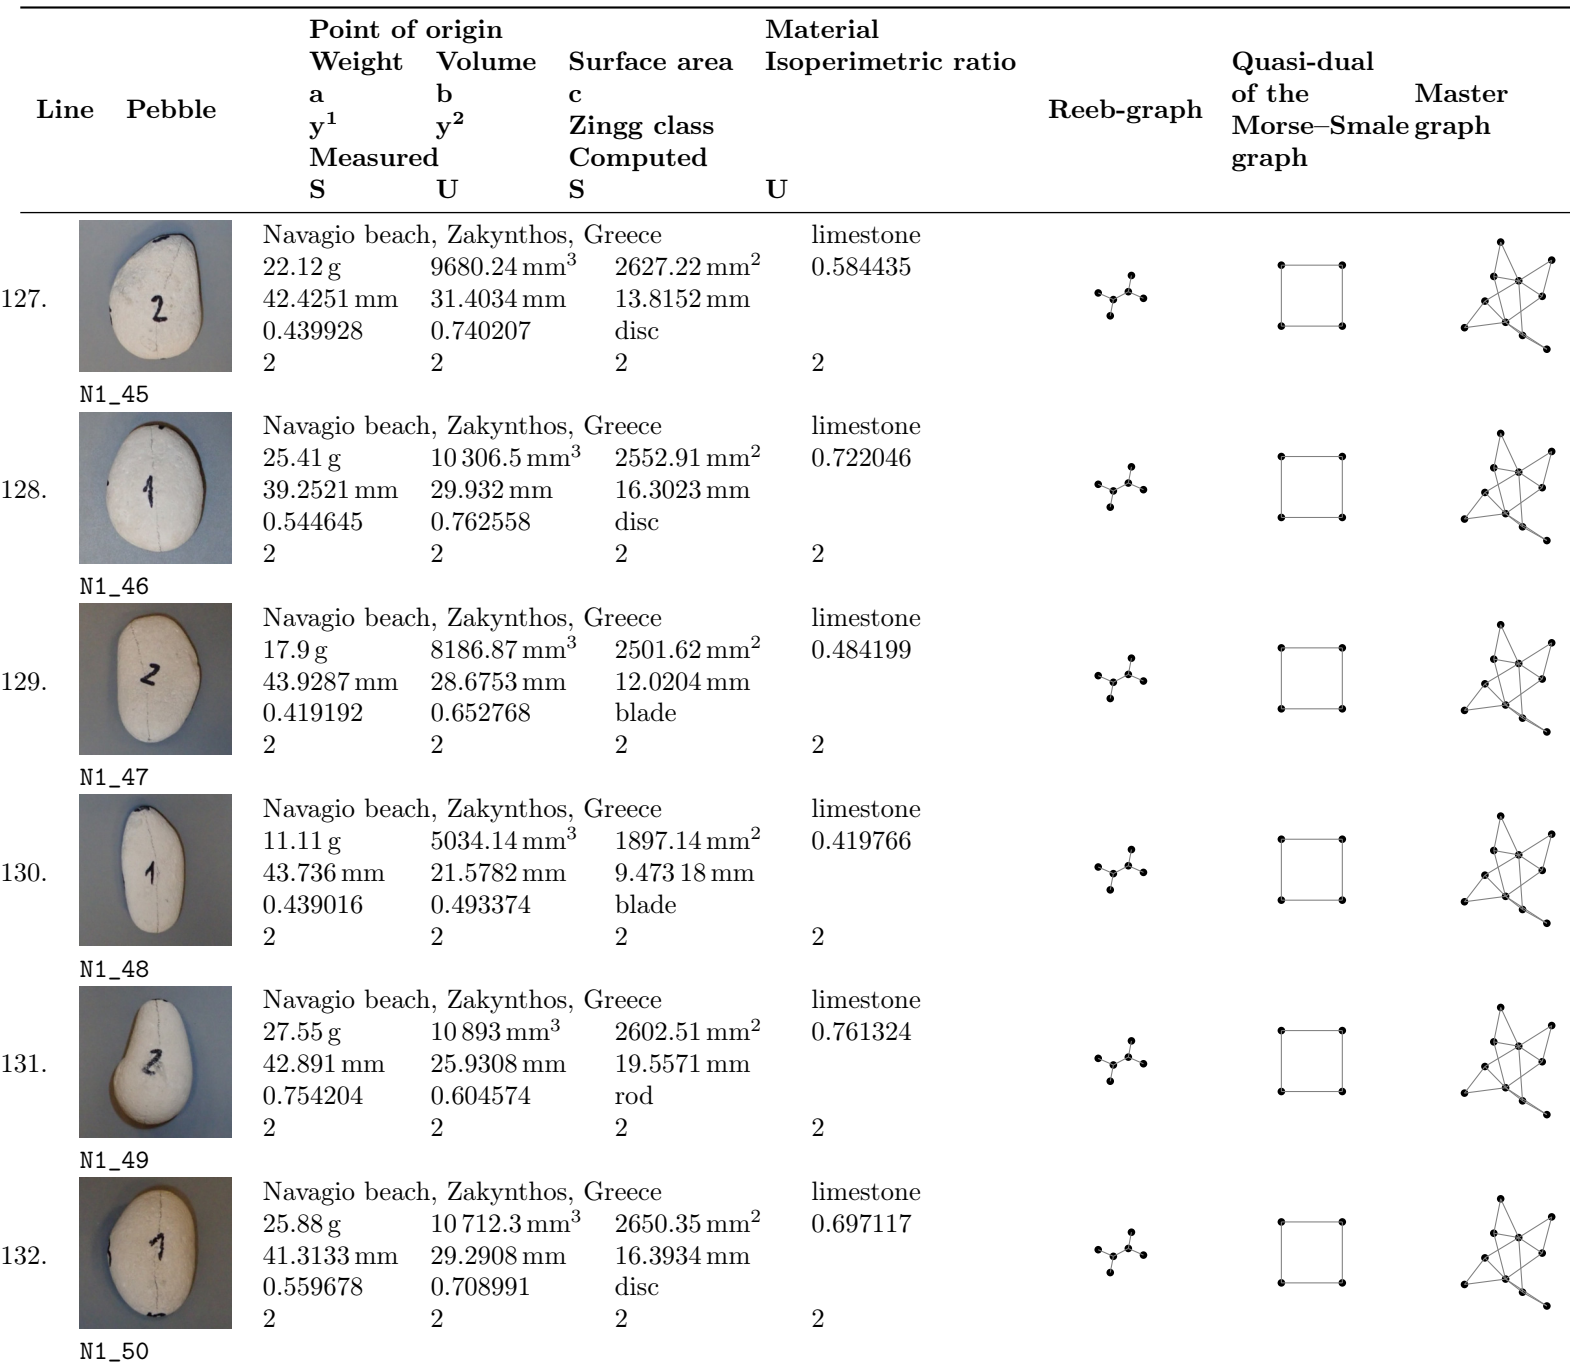  | 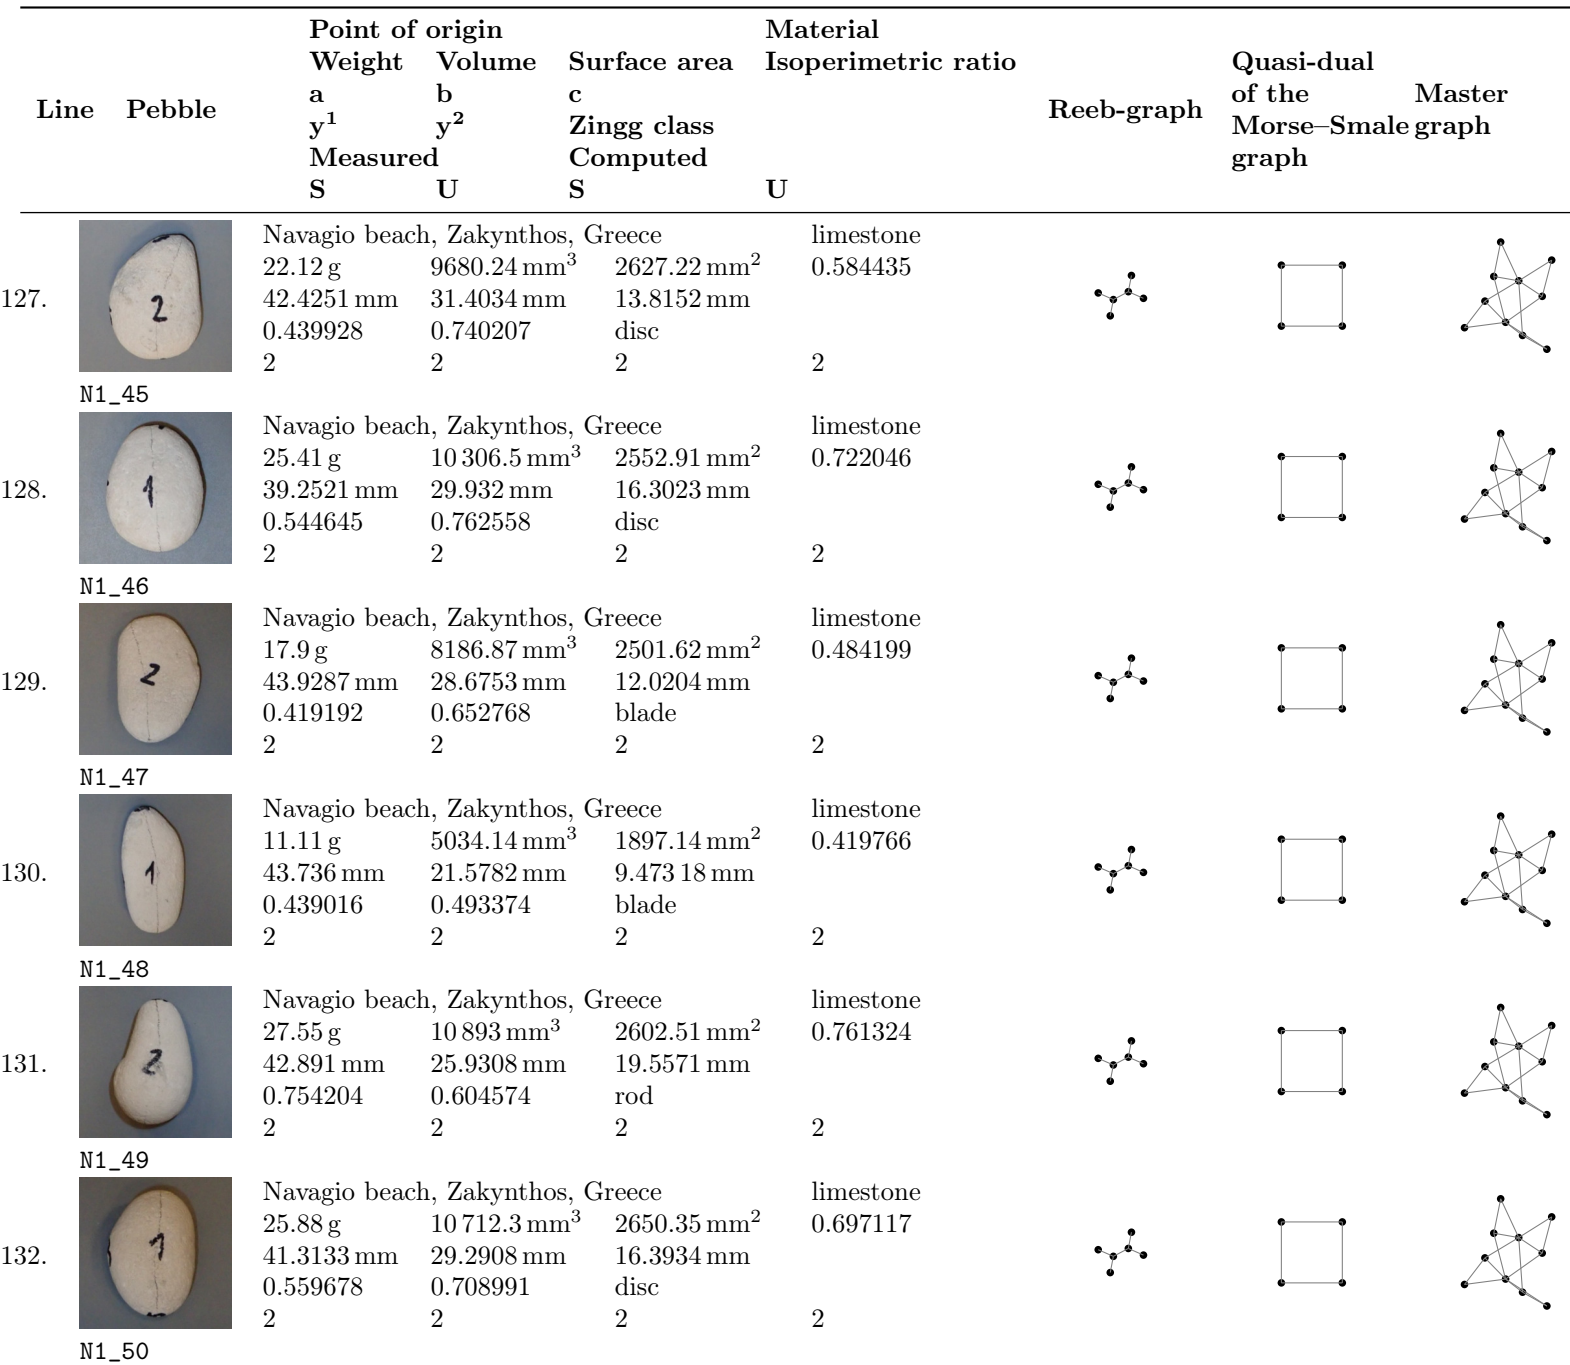  |                 |
| N1_48 |                                                                                     |                                                                            |                                                         |                                                      |                                |                                                                                       |                                                                                       |                                                                                       |                 |
| 131.  | 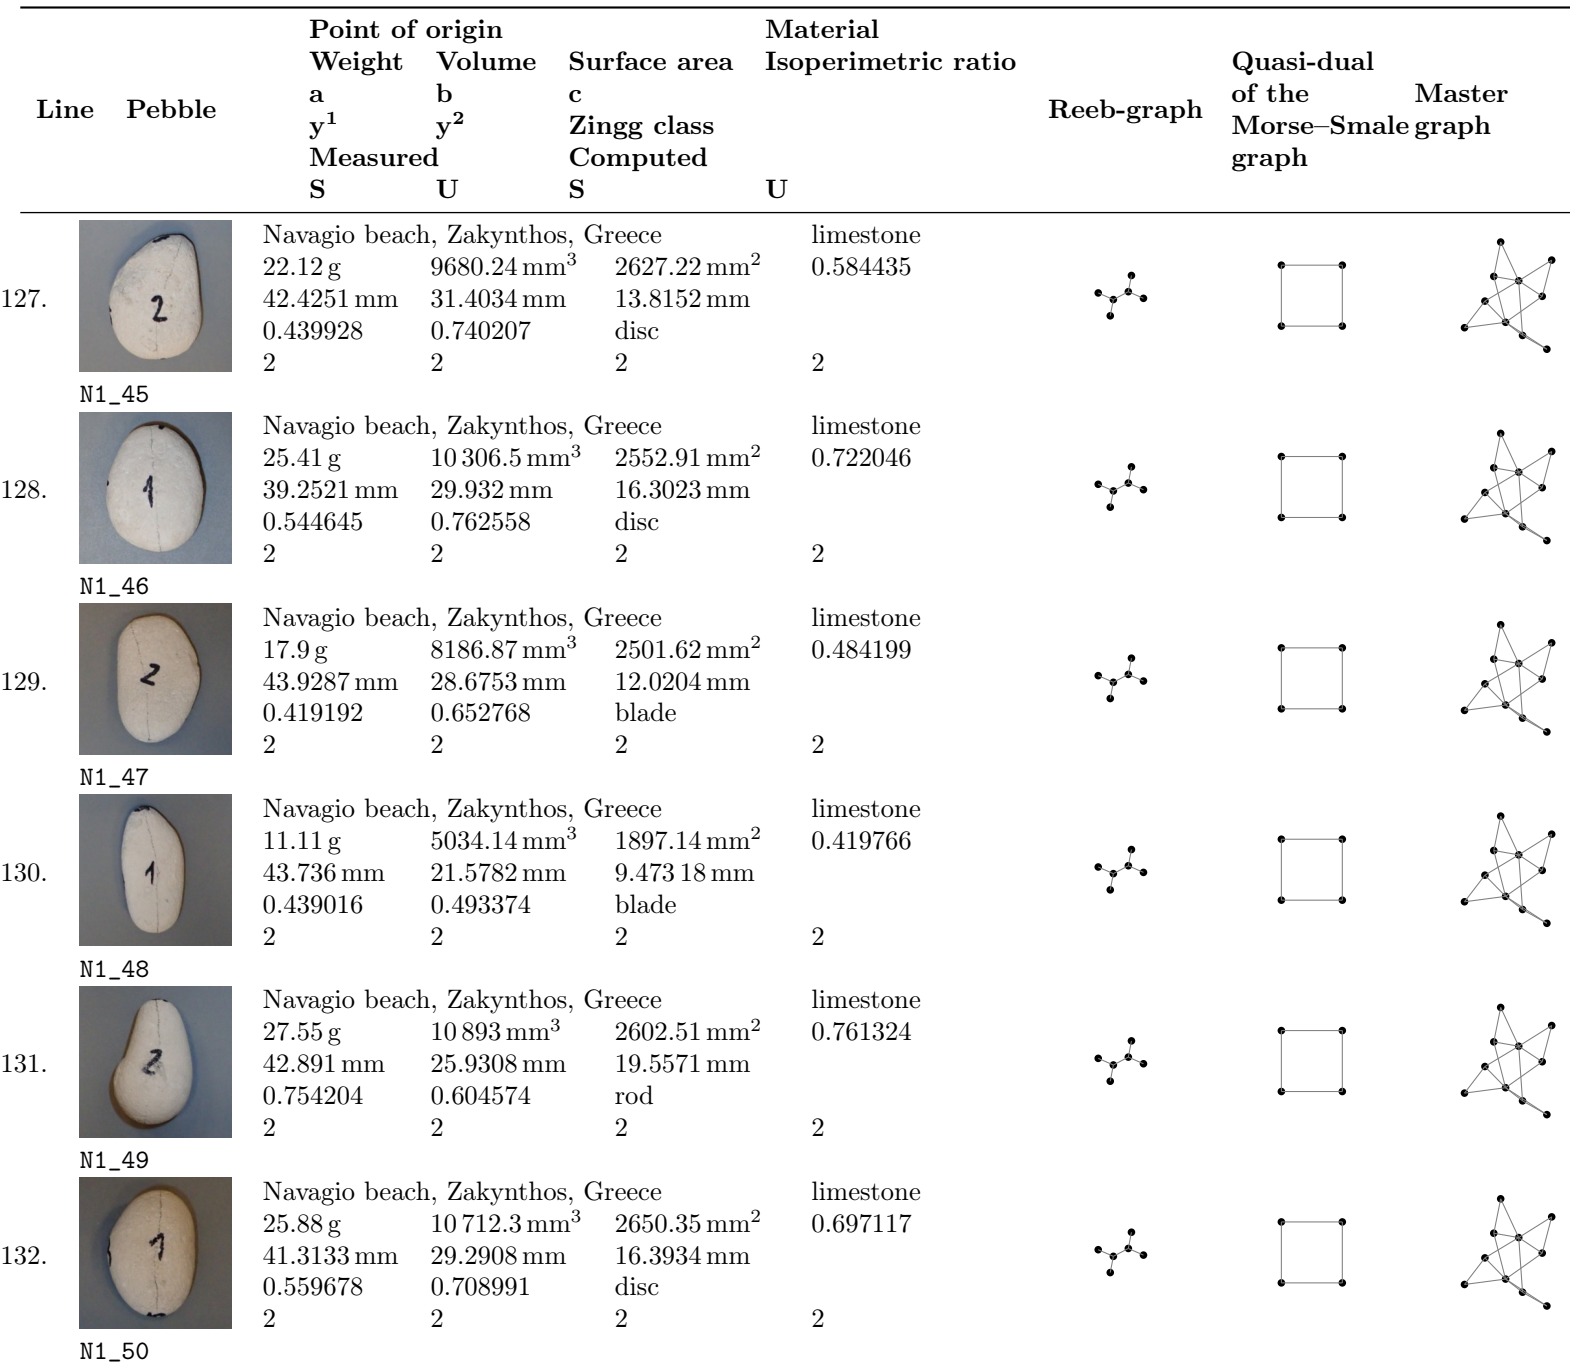 | Navagio beach, Zakynthos, Greece<br>27.55 g<br>42.891 mm<br>0.754204<br>2  | 10 893 mm <sup>3</sup><br>25.9308 mm<br>0.604574<br>2   | 2602.51 mm <sup>2</sup><br>19.5571 mm<br>rod<br>2    | limestone<br>0.761324<br><br>2 | 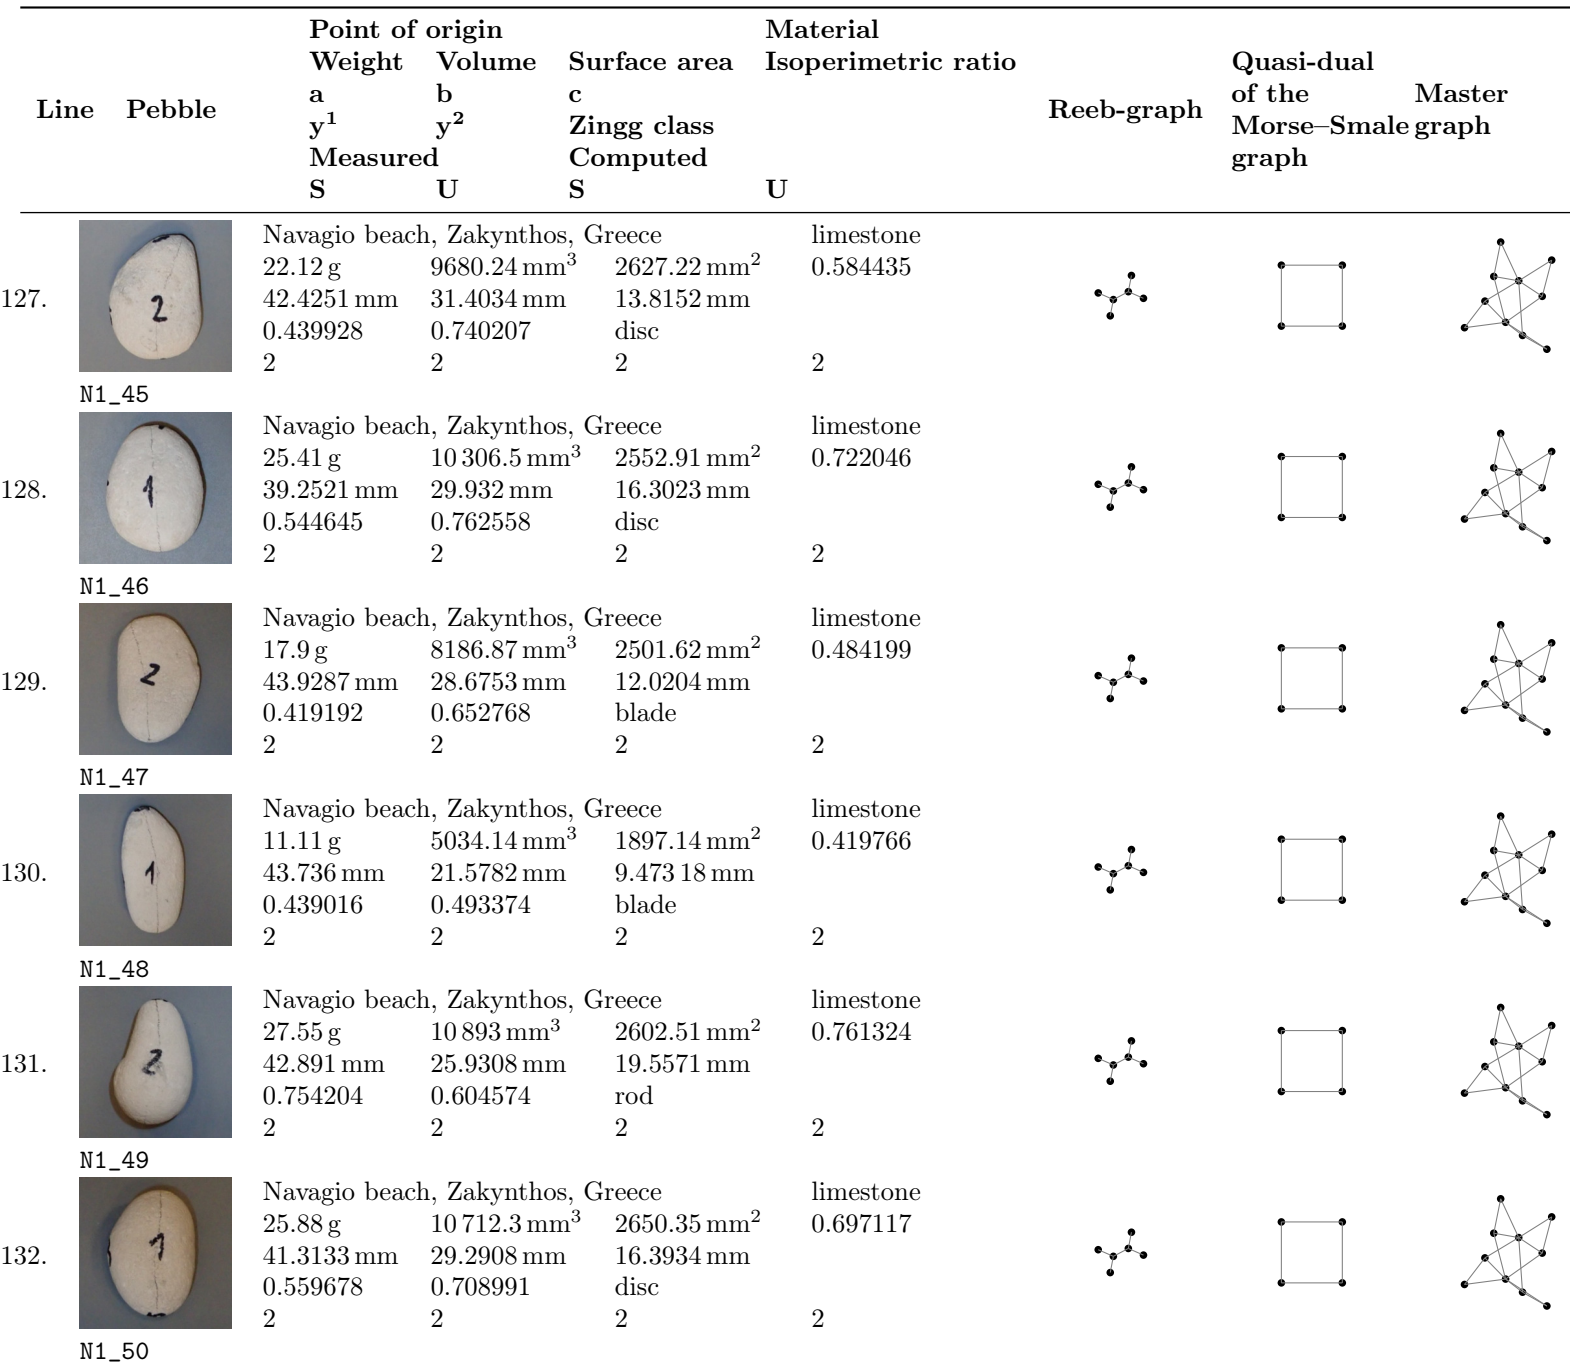 | 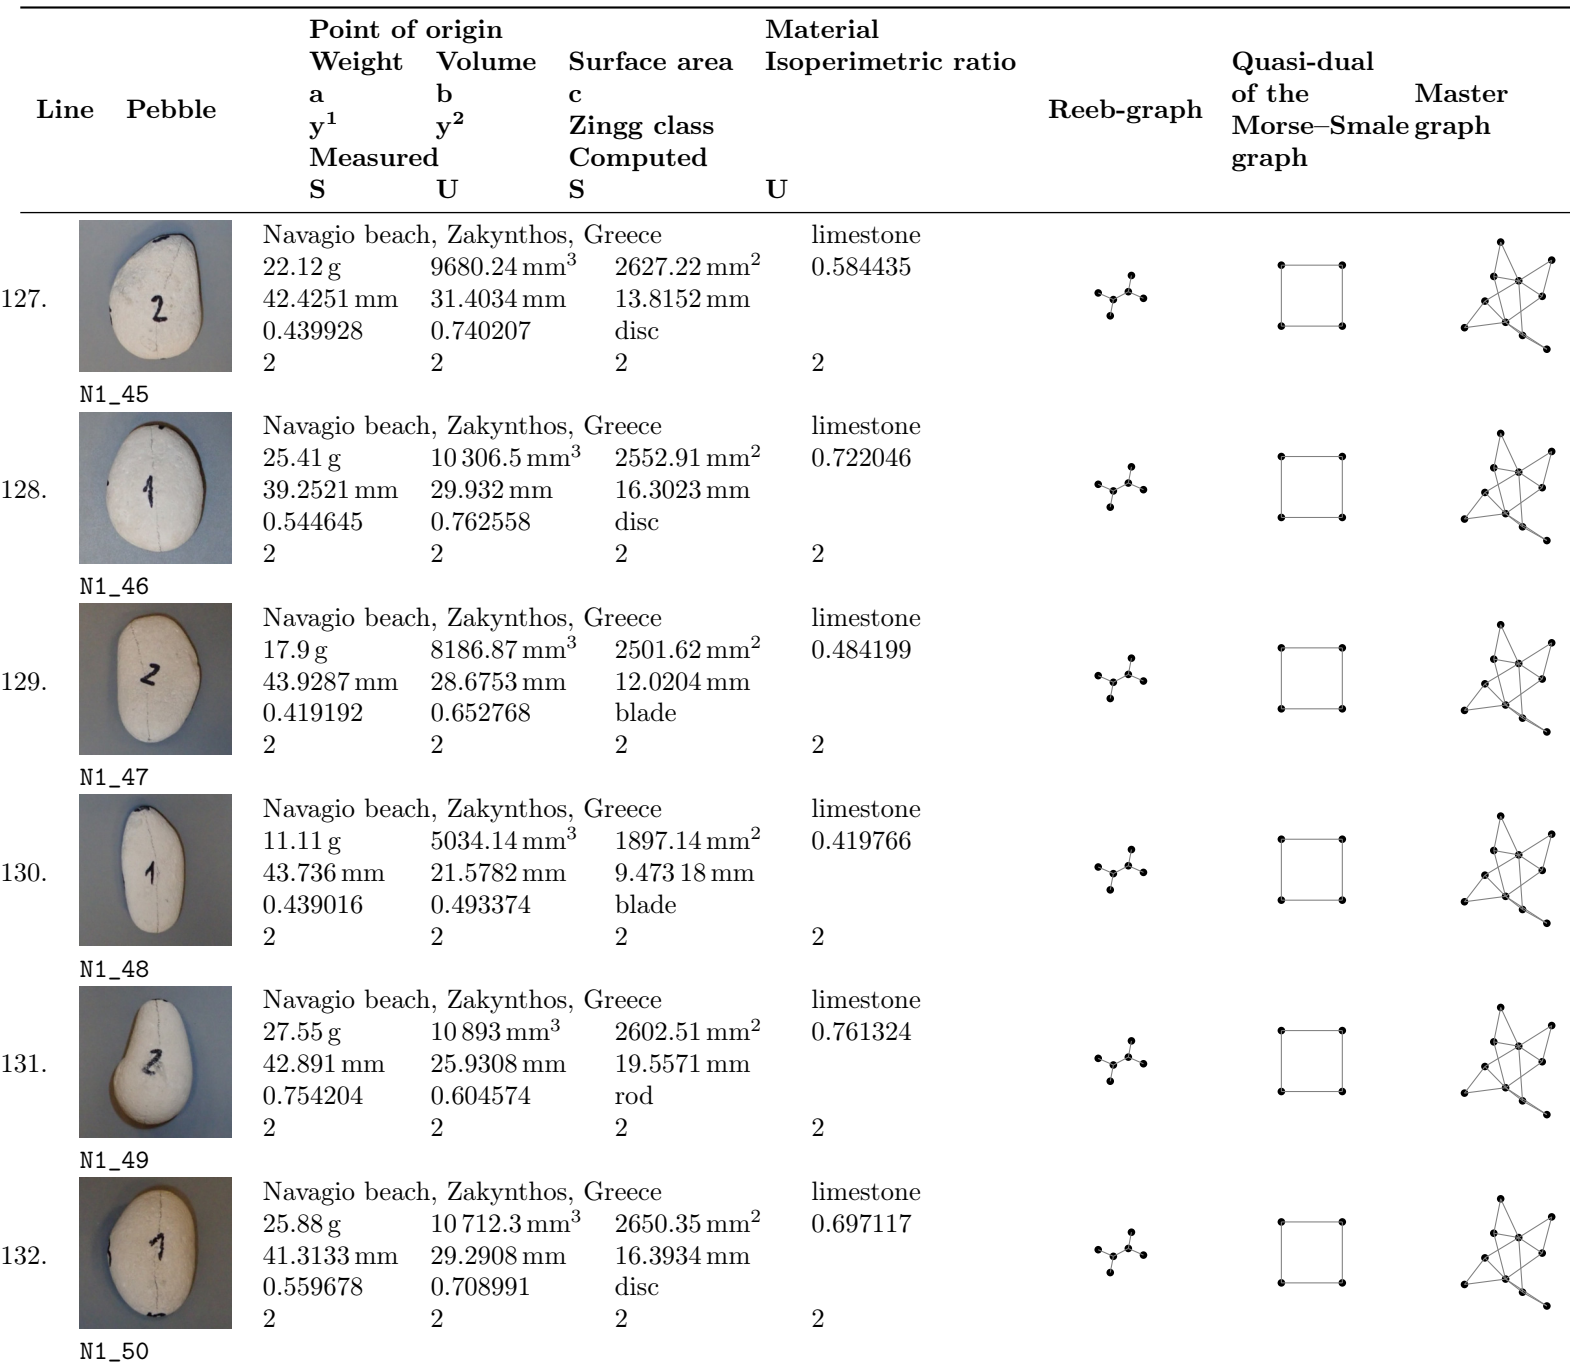 | 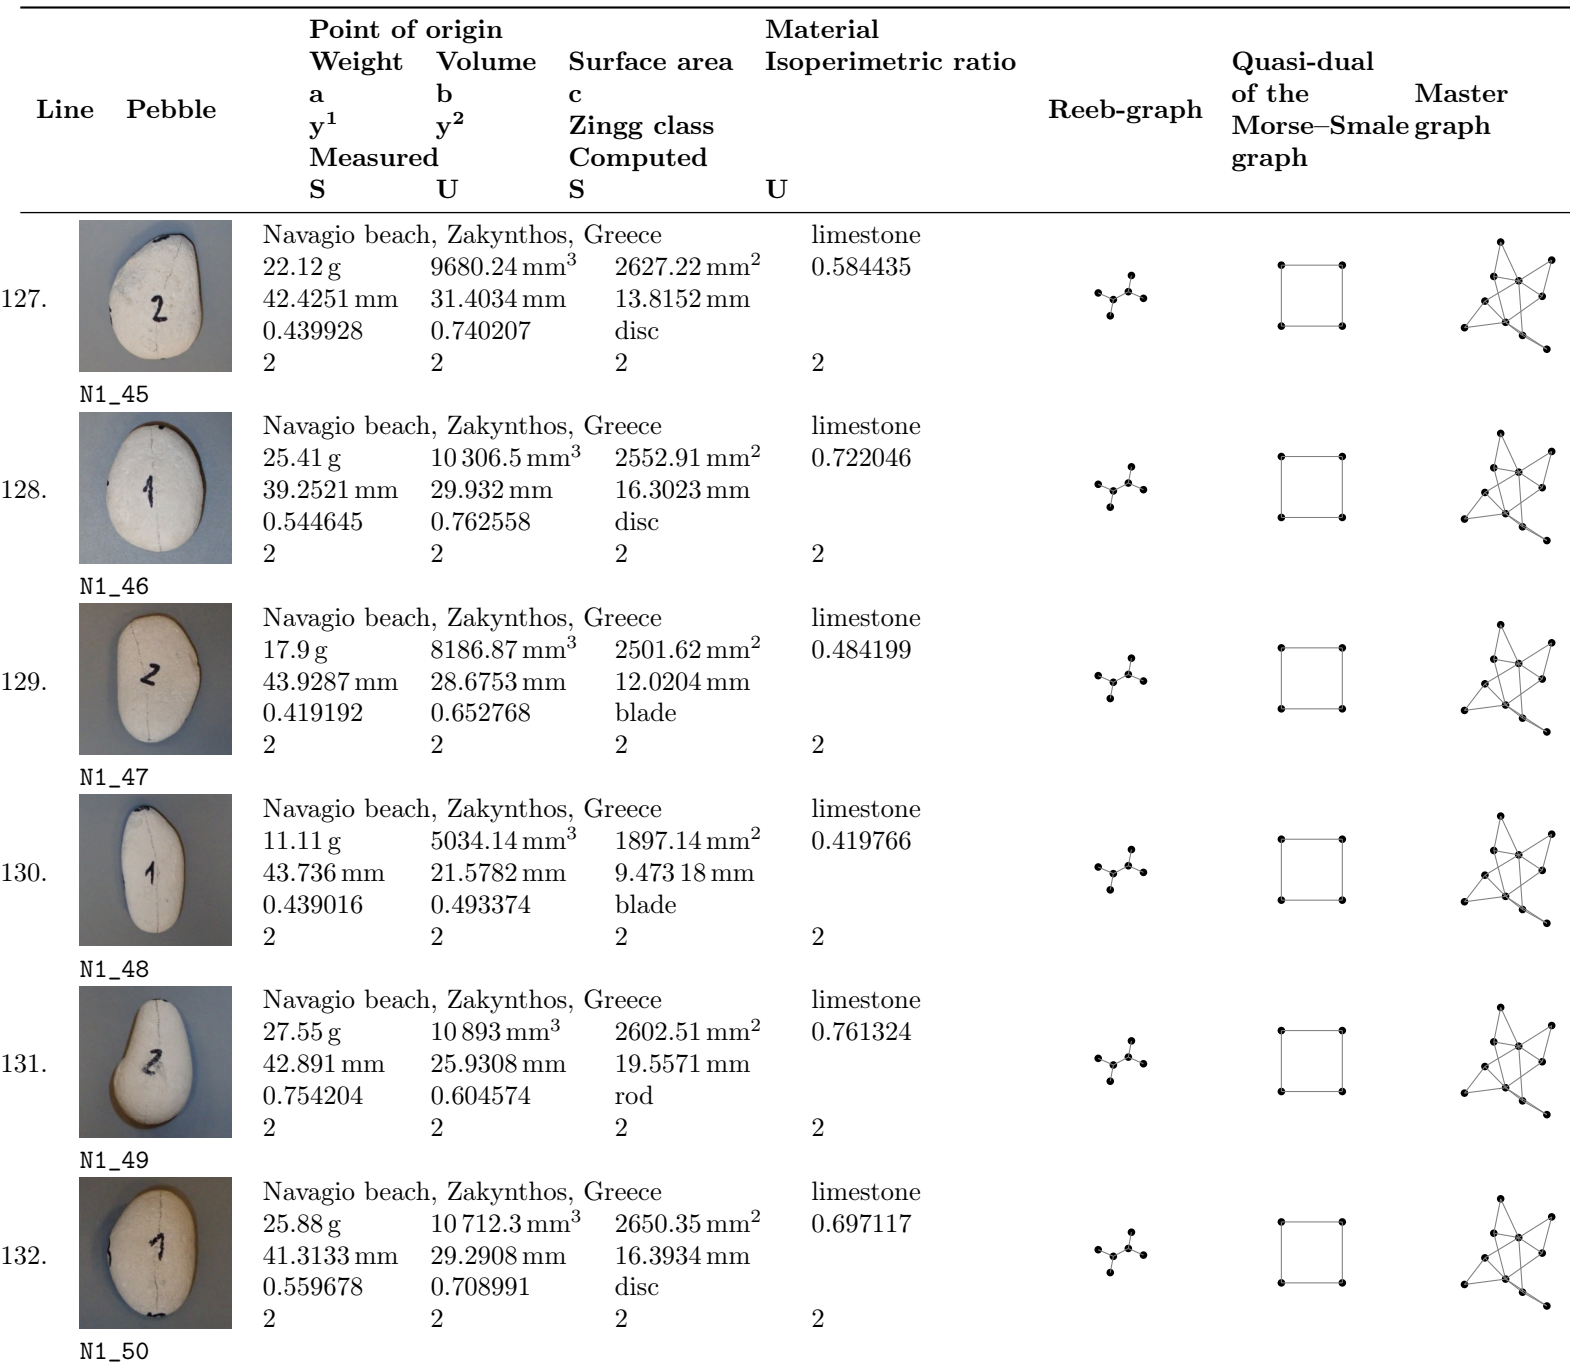 |                 |
| N1_49 |                                                                                     |                                                                            |                                                         |                                                      |                                |                                                                                       |                                                                                       |                                                                                       |                 |
| 132.  | 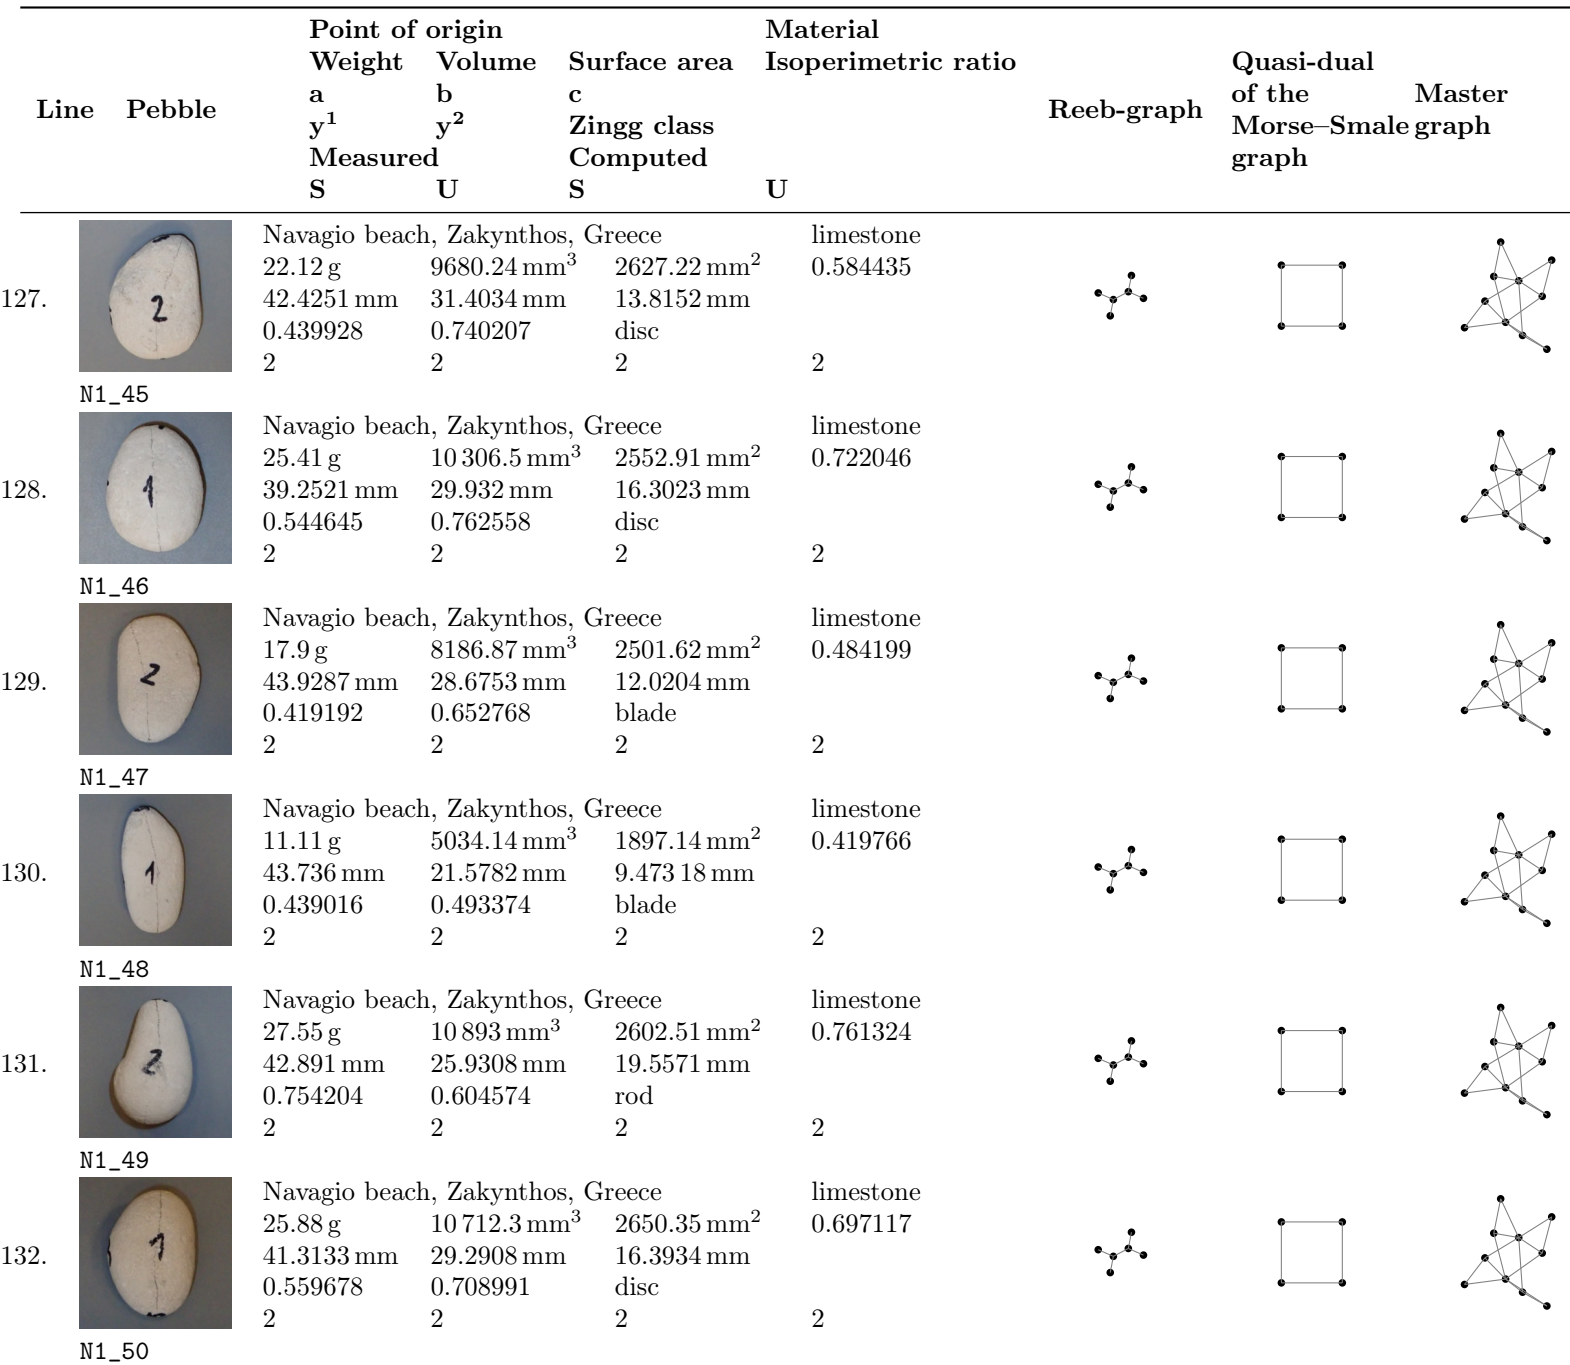 | Navagio beach, Zakynthos, Greece<br>25.88 g<br>41.3133 mm<br>0.559678<br>2 | 10 712.3 mm <sup>3</sup><br>29.2908 mm<br>0.708991<br>2 | 2650.35 mm <sup>2</sup><br>16.3934 mm<br>disc<br>2   | limestone<br>0.697117<br><br>2 | 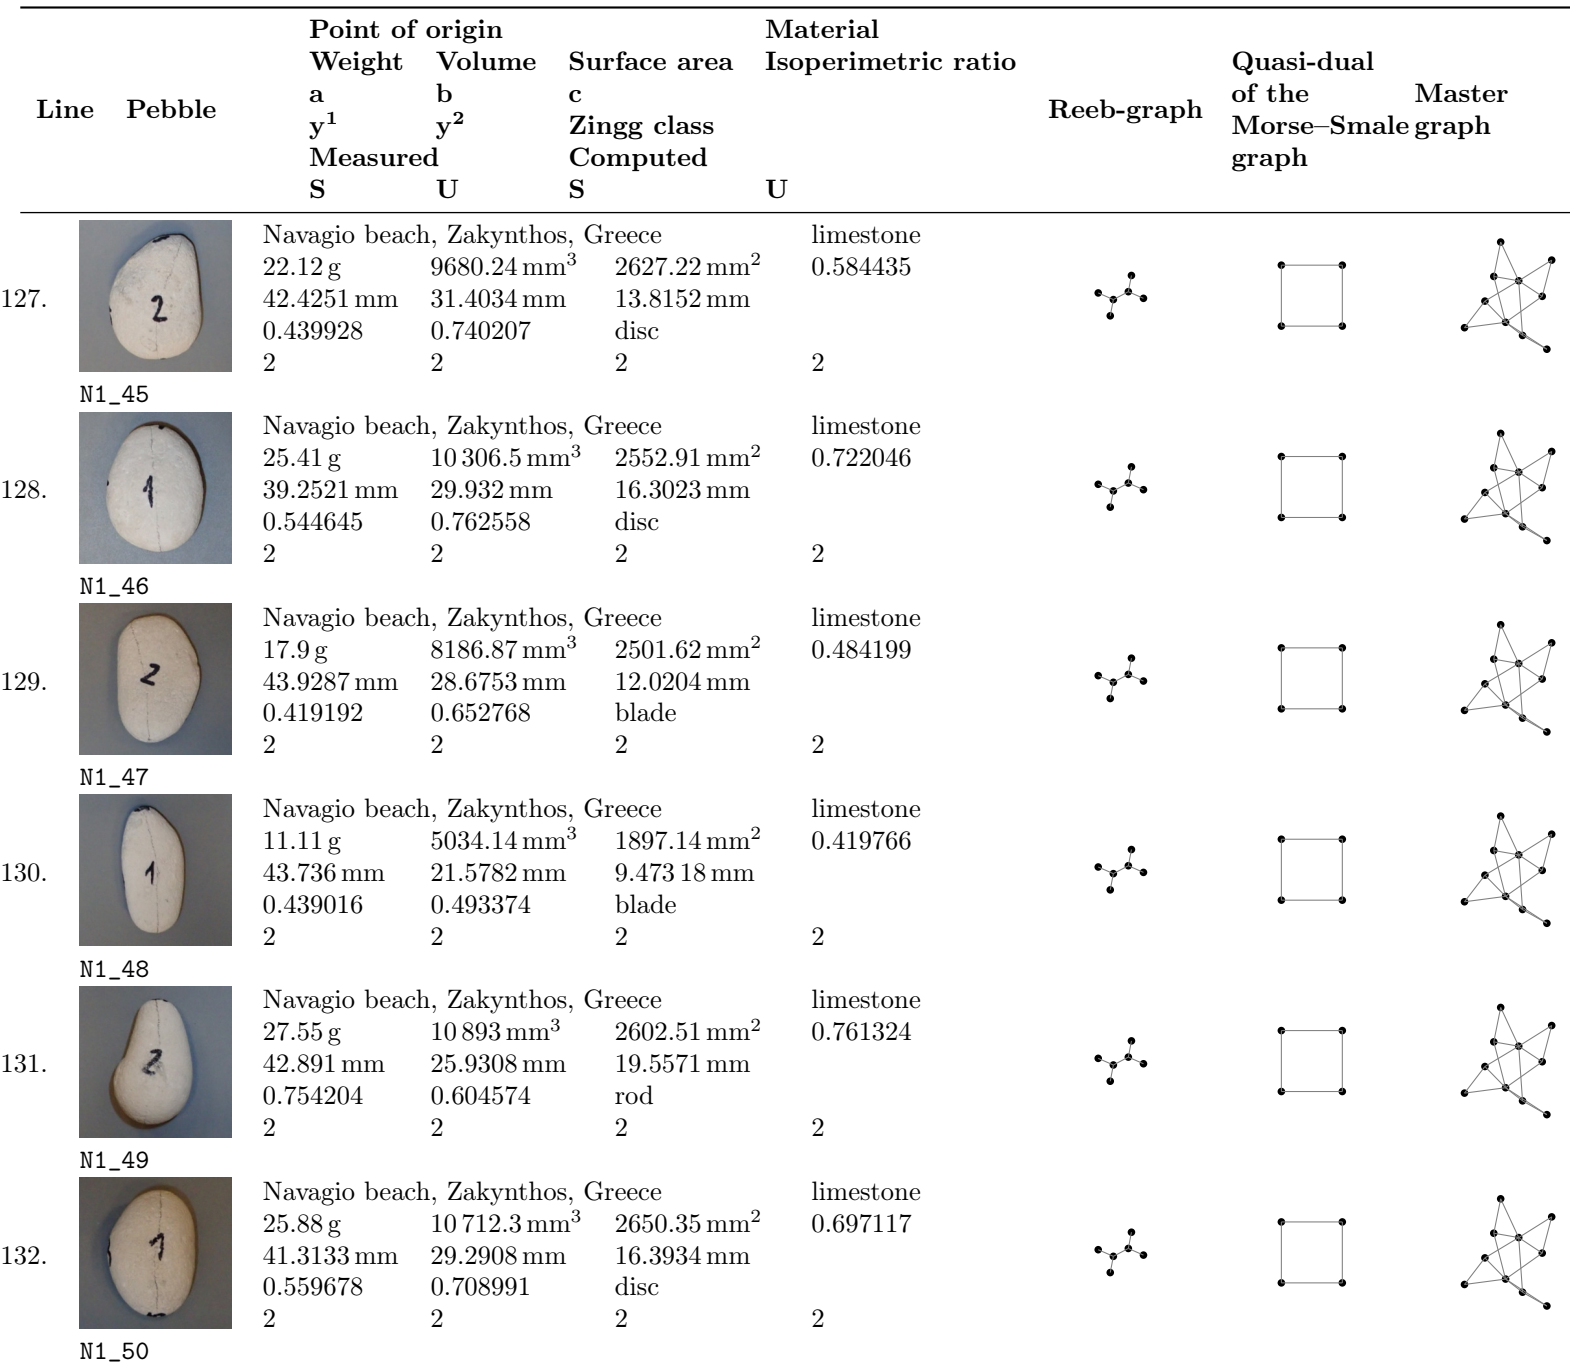 | 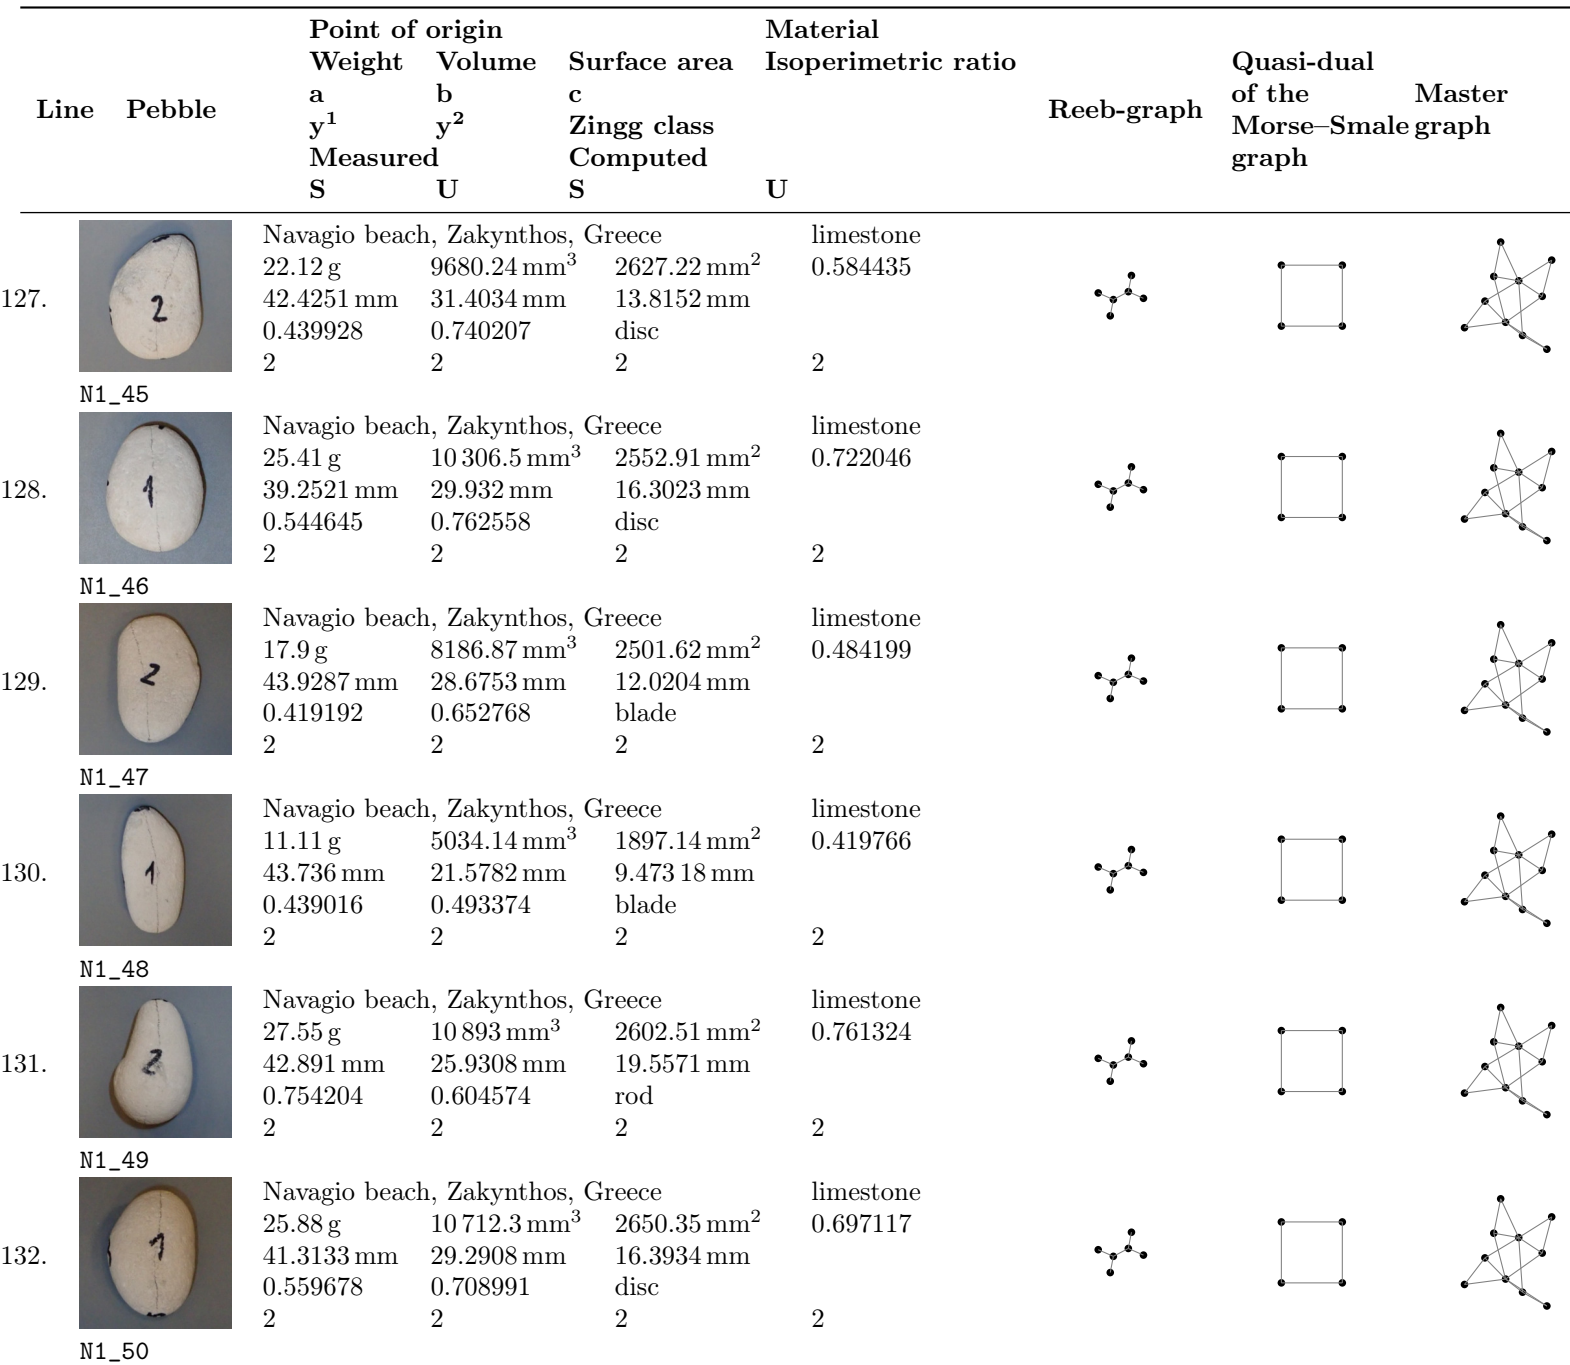 | 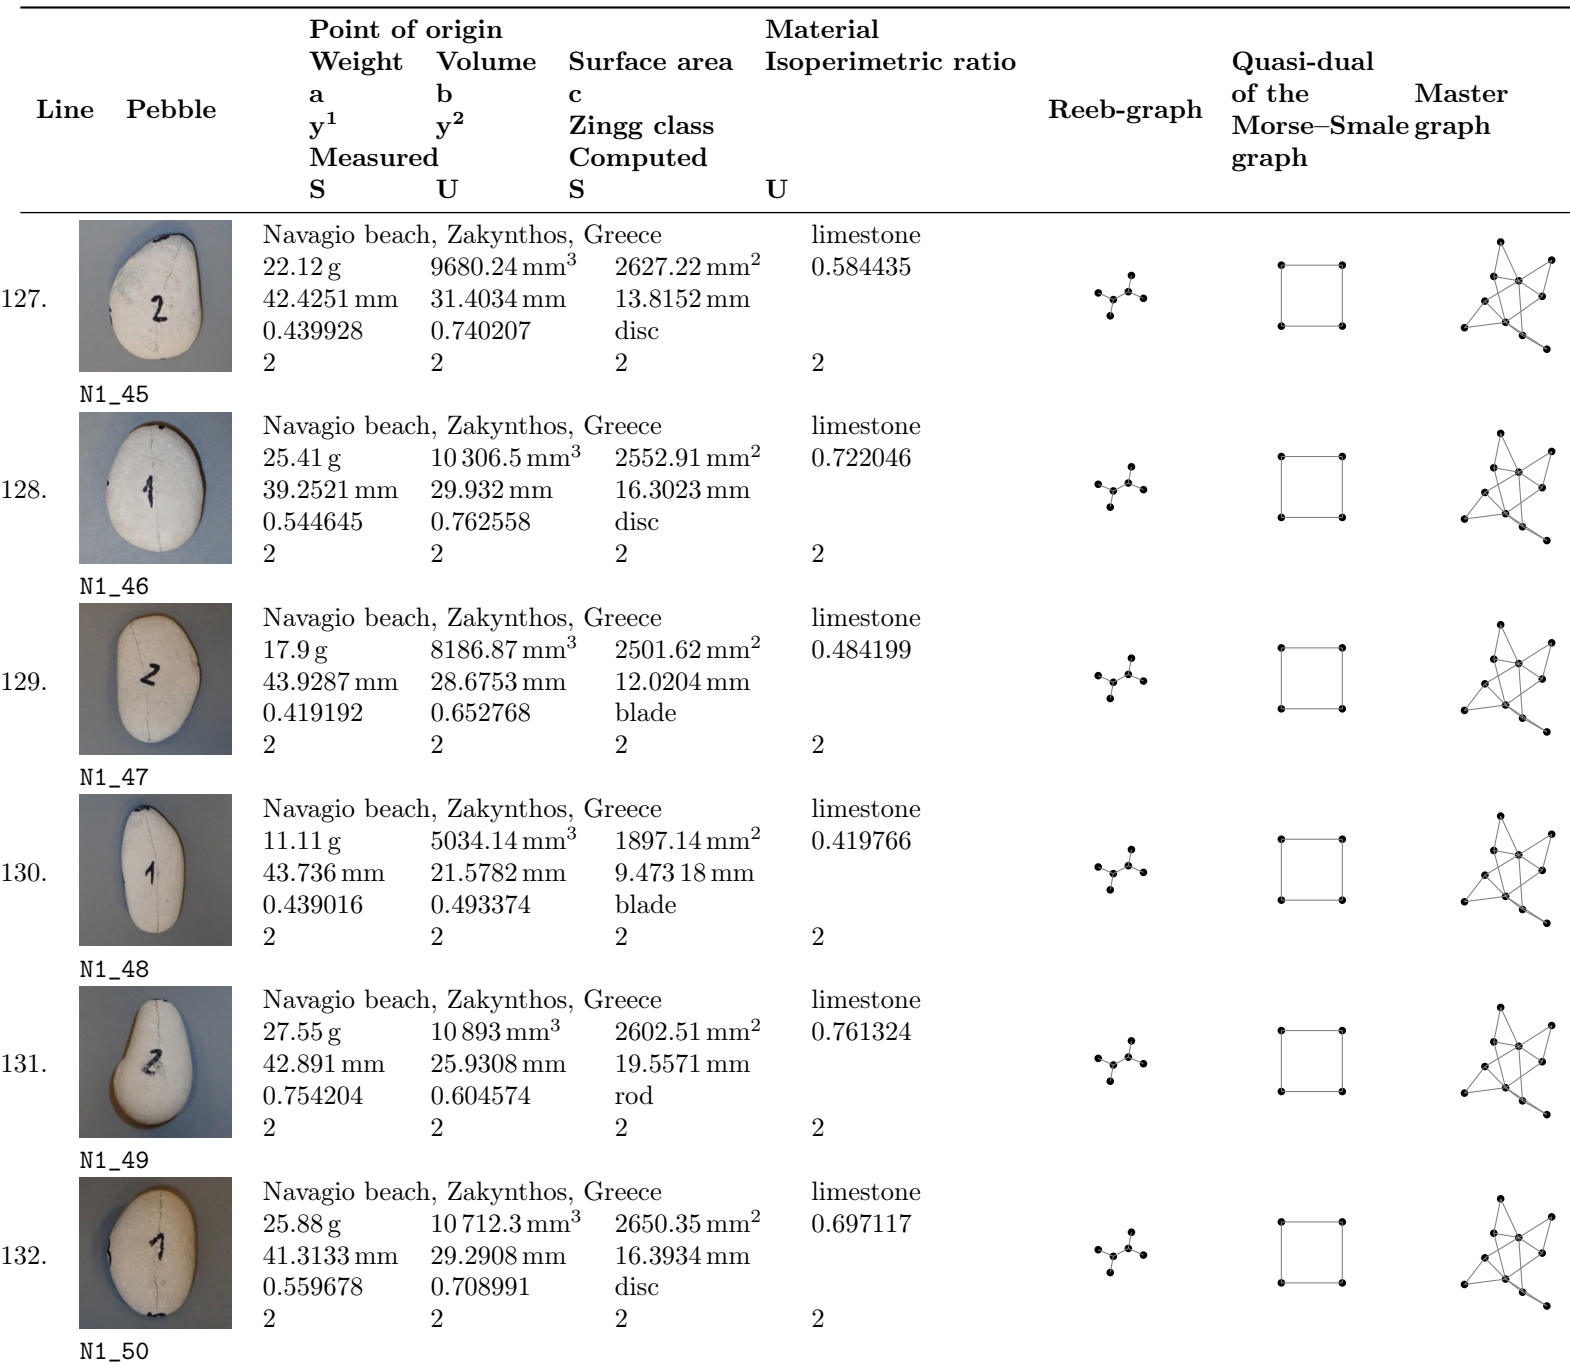 |                 |
| N1_50 |                                                                                     |                                                                            |                                                         |                                                      |                                |                                                                                       |                                                                                       |                                                                                       |                 |

| Line | Pebble                                                                              | Point of origin                  |                          |                              | Material              | Reeb-graph                                                                            | Quasi-dual<br>of the<br>Morse–Smale<br>graph                                          | Master<br>graph                                                                       |
|------|-------------------------------------------------------------------------------------|----------------------------------|--------------------------|------------------------------|-----------------------|---------------------------------------------------------------------------------------|---------------------------------------------------------------------------------------|---------------------------------------------------------------------------------------|
|      |                                                                                     | Weight                           | Volume                   | Surface area                 |                       |                                                                                       |                                                                                       |                                                                                       |
|      |                                                                                     | a                                | b                        | c                            |                       |                                                                                       |                                                                                       |                                                                                       |
|      |                                                                                     | y <sup>1</sup><br>Measured<br>S  | y <sup>2</sup><br>U      | Zingg class<br>Computed<br>S |                       |                                                                                       |                                                                                       |                                                                                       |
| 133. | 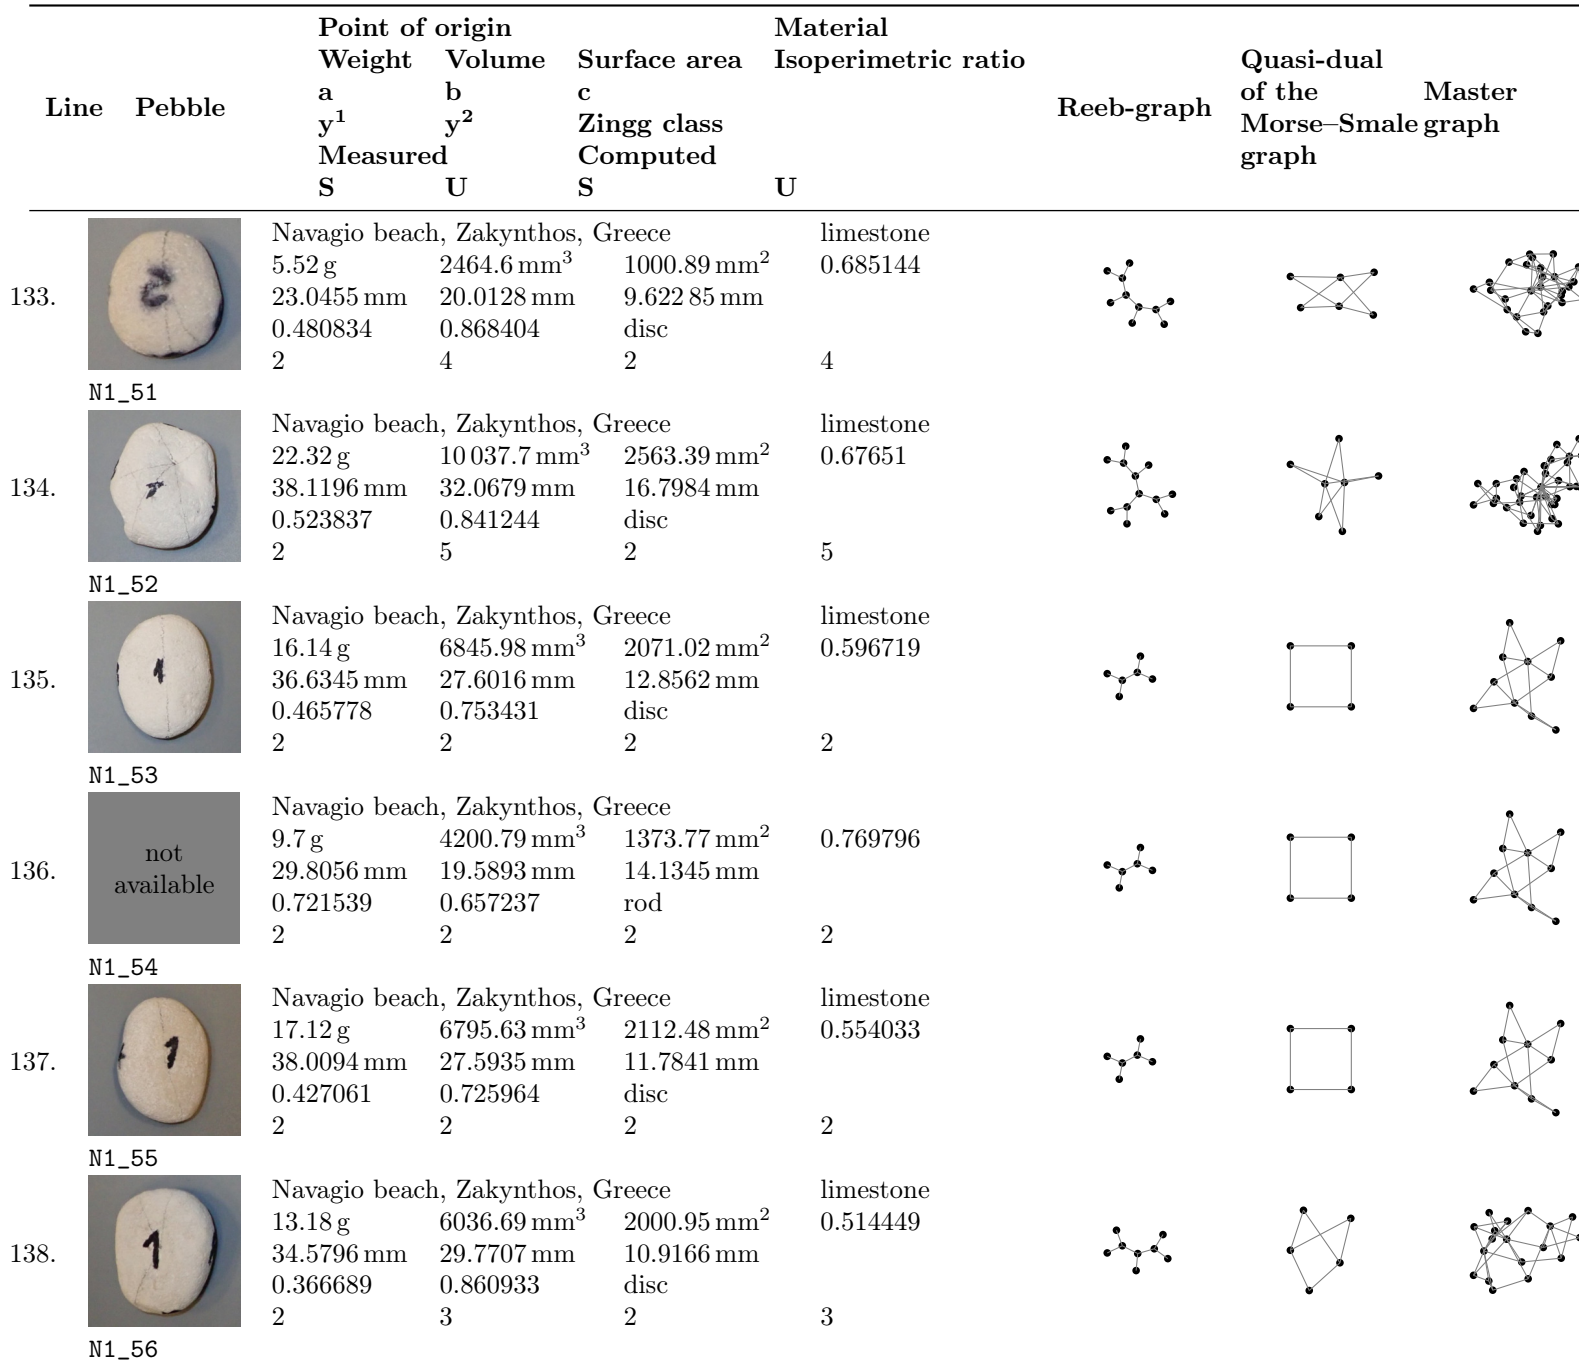   | Navagio beach, Zakynthos, Greece |                          |                              | limestone<br>0.685144 | 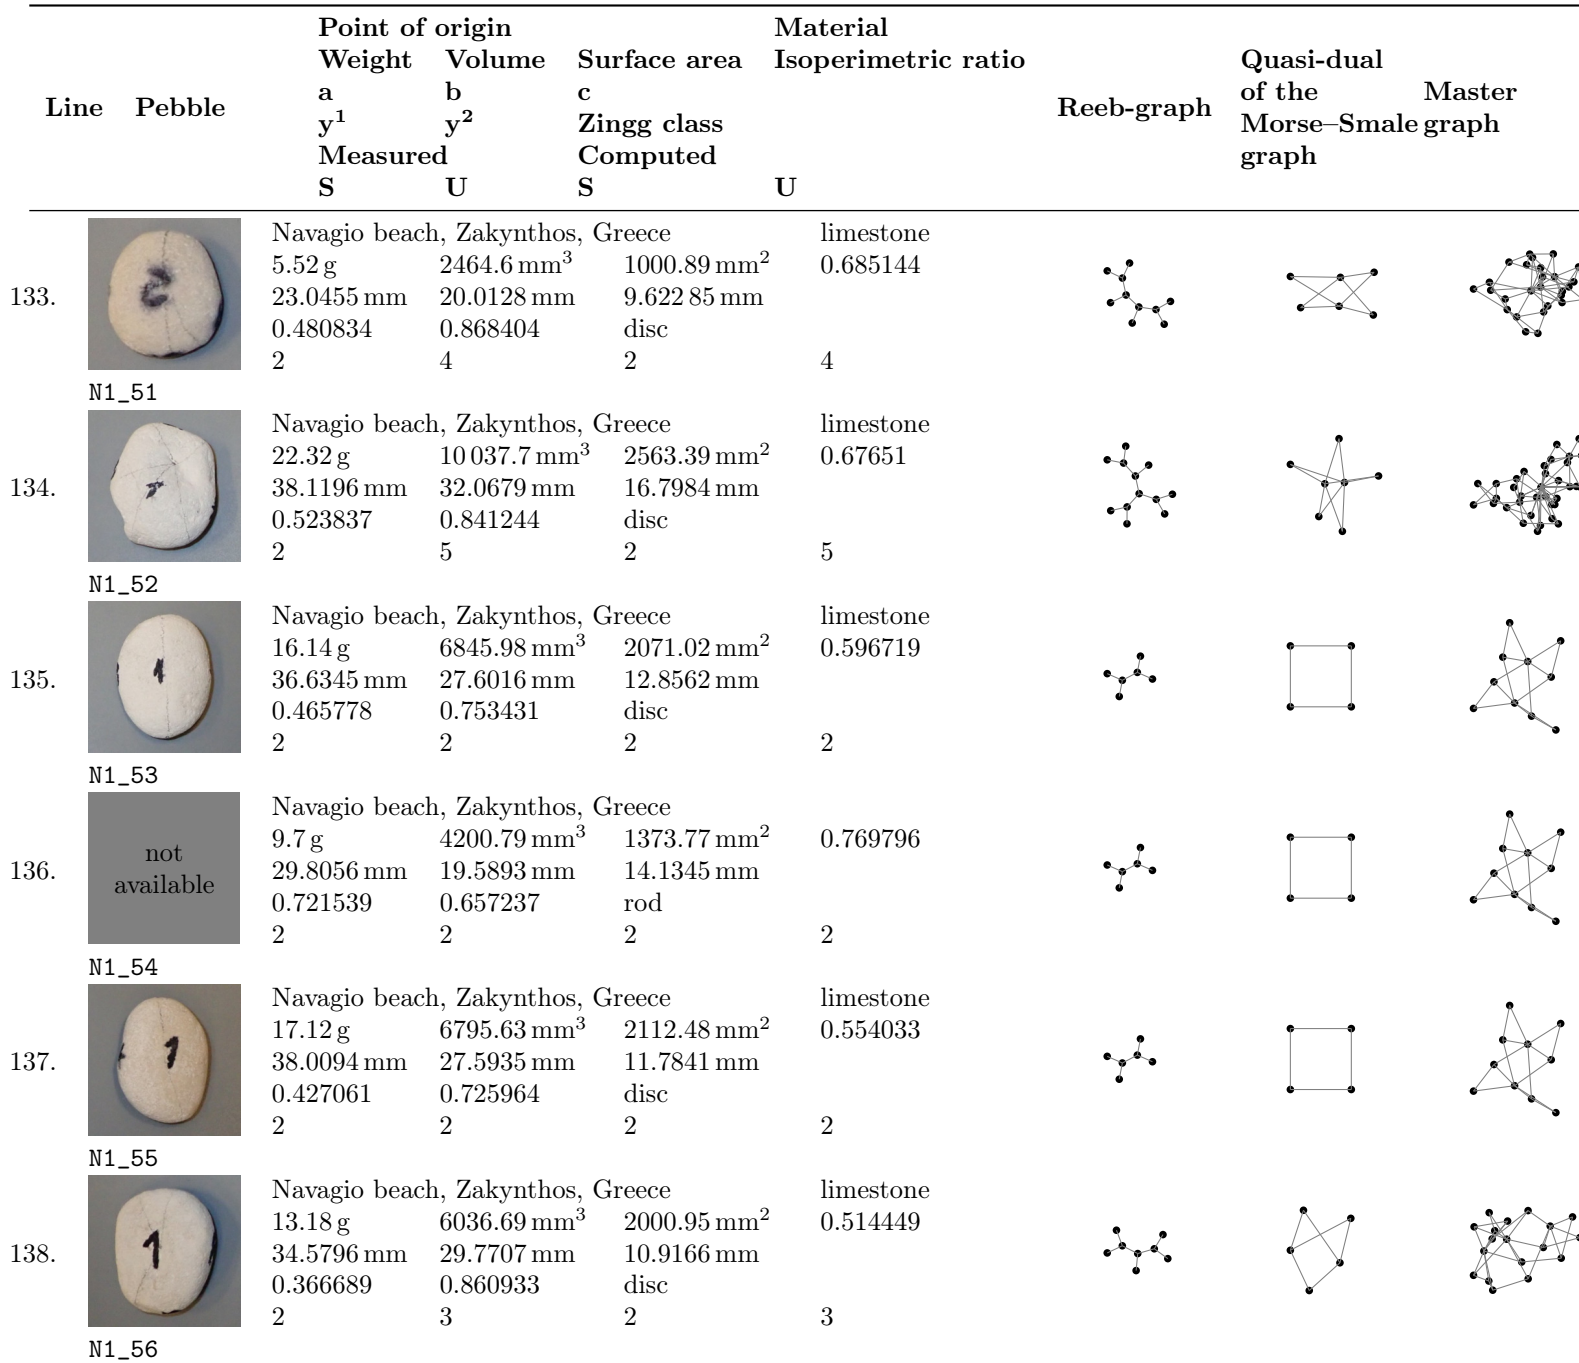   | 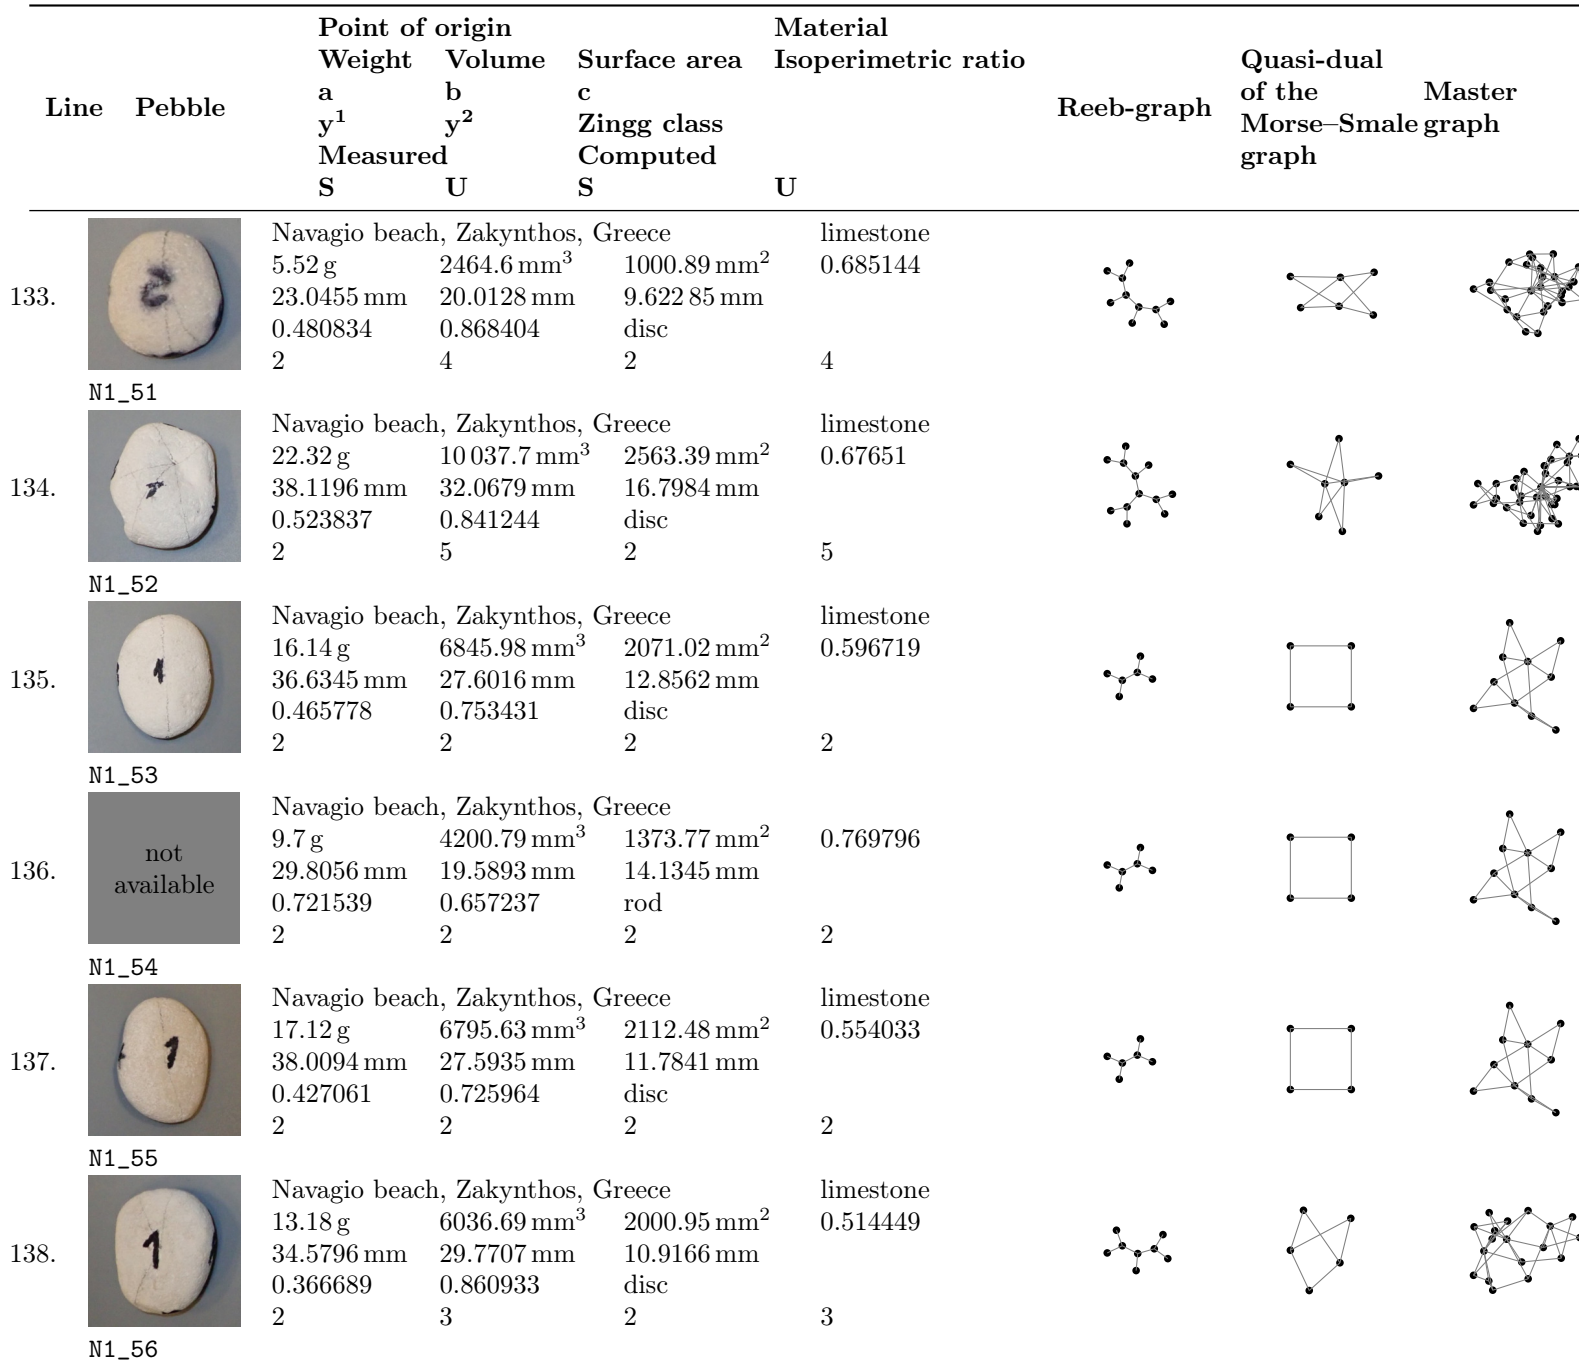   | 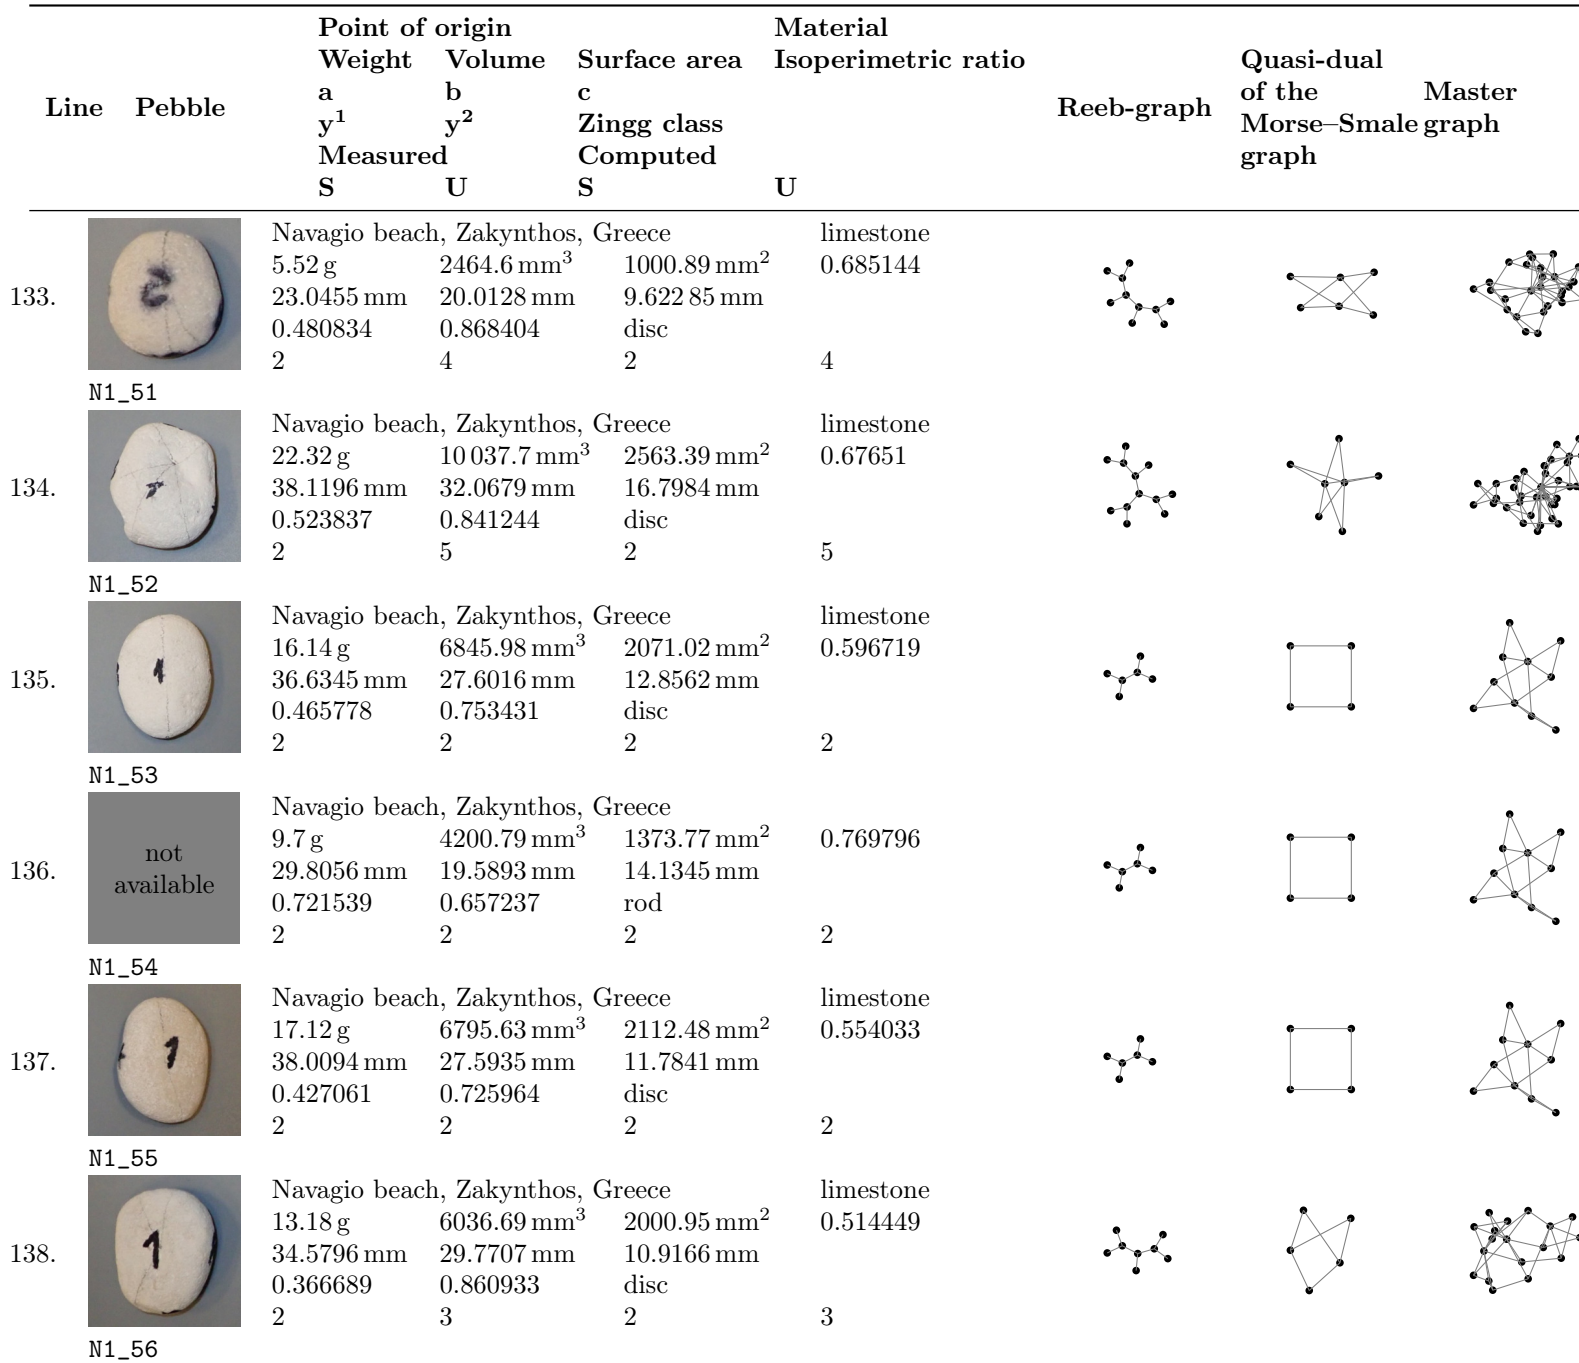   |
|      |                                                                                     | 5.52 g                           | 2464.6 mm <sup>3</sup>   | 1000.89 mm <sup>2</sup>      |                       |                                                                                       |                                                                                       |                                                                                       |
|      |                                                                                     | 23.0455 mm                       | 20.0128 mm               | 9.622 85 mm                  |                       |                                                                                       |                                                                                       |                                                                                       |
|      |                                                                                     | 0.480834                         | 0.868404                 | disc                         |                       |                                                                                       |                                                                                       |                                                                                       |
|      | N1_51                                                                               | 2                                | 4                        | 2                            | 4                     |                                                                                       |                                                                                       |                                                                                       |
| 134. | 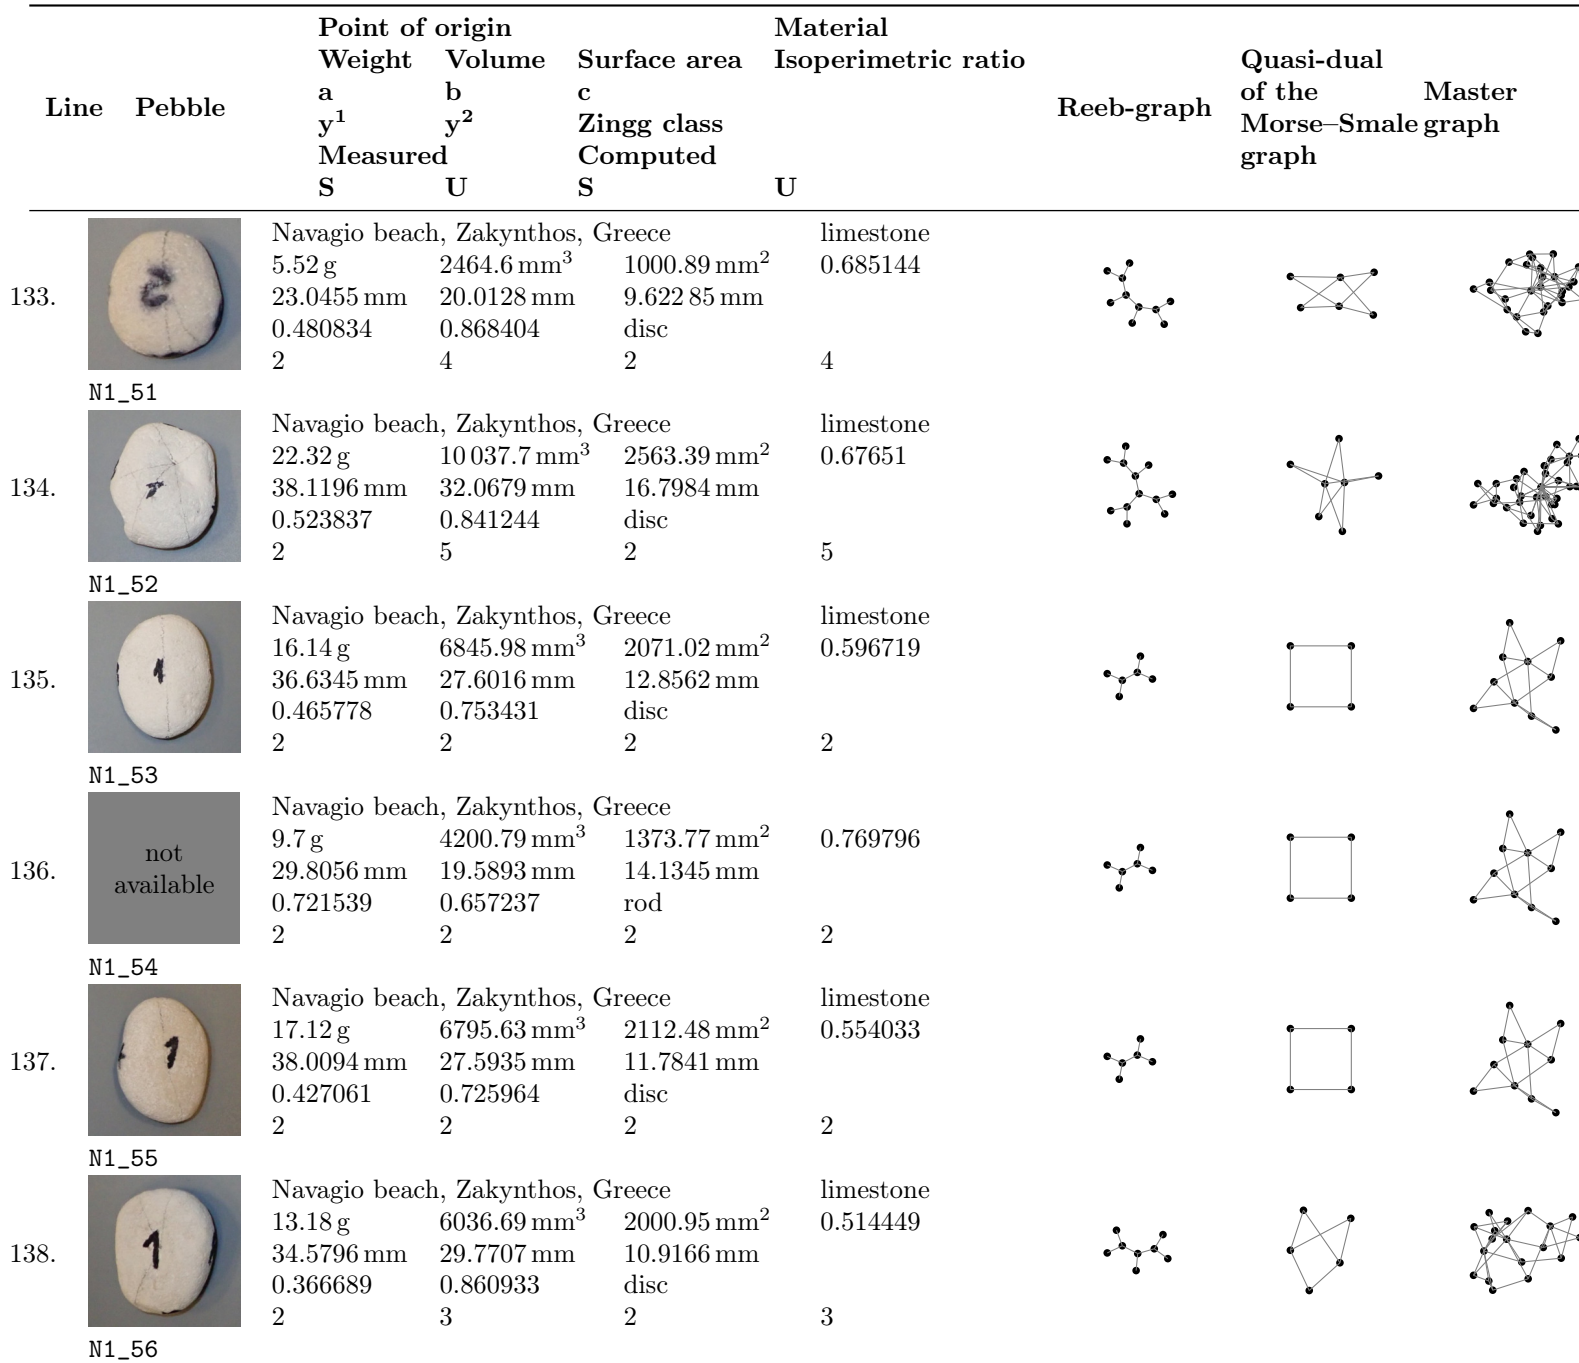   | Navagio beach, Zakynthos, Greece |                          |                              | limestone<br>0.67651  | 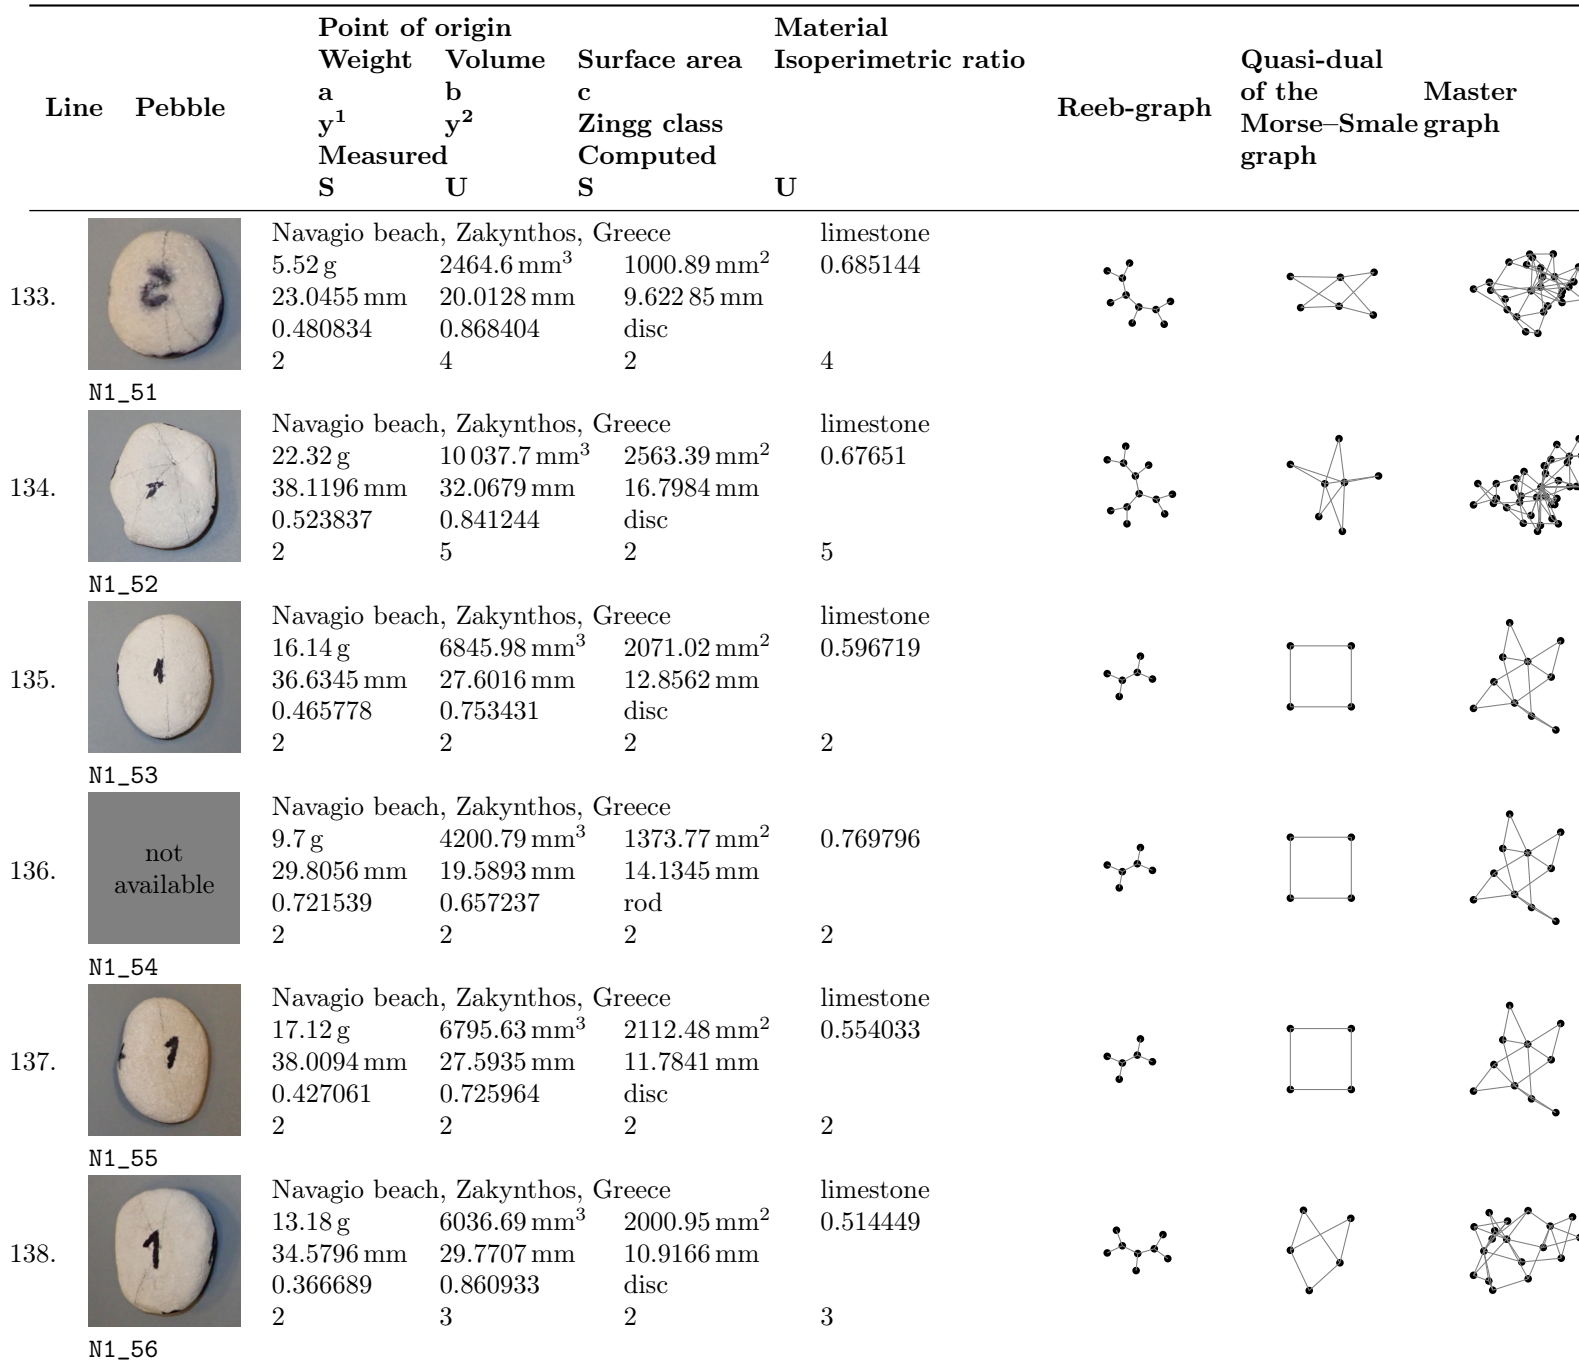   | 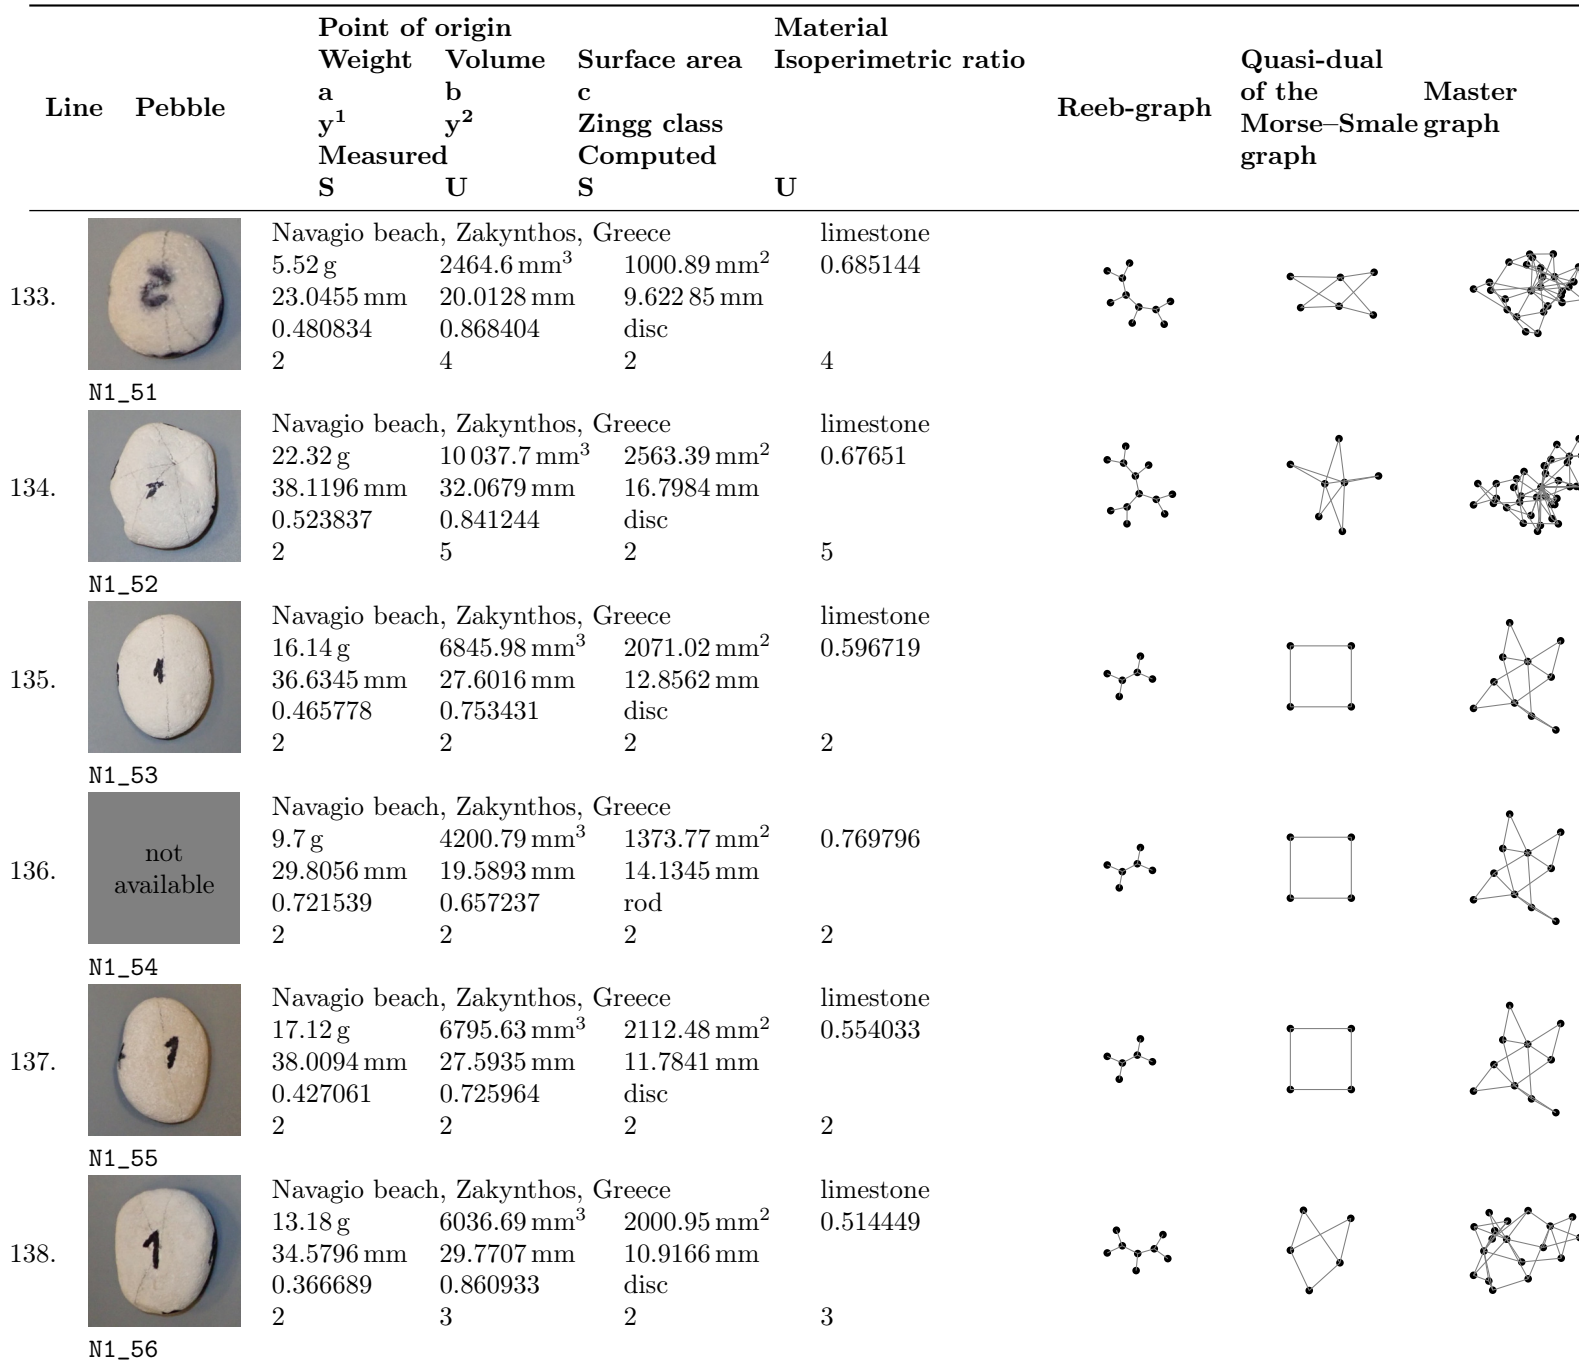   | 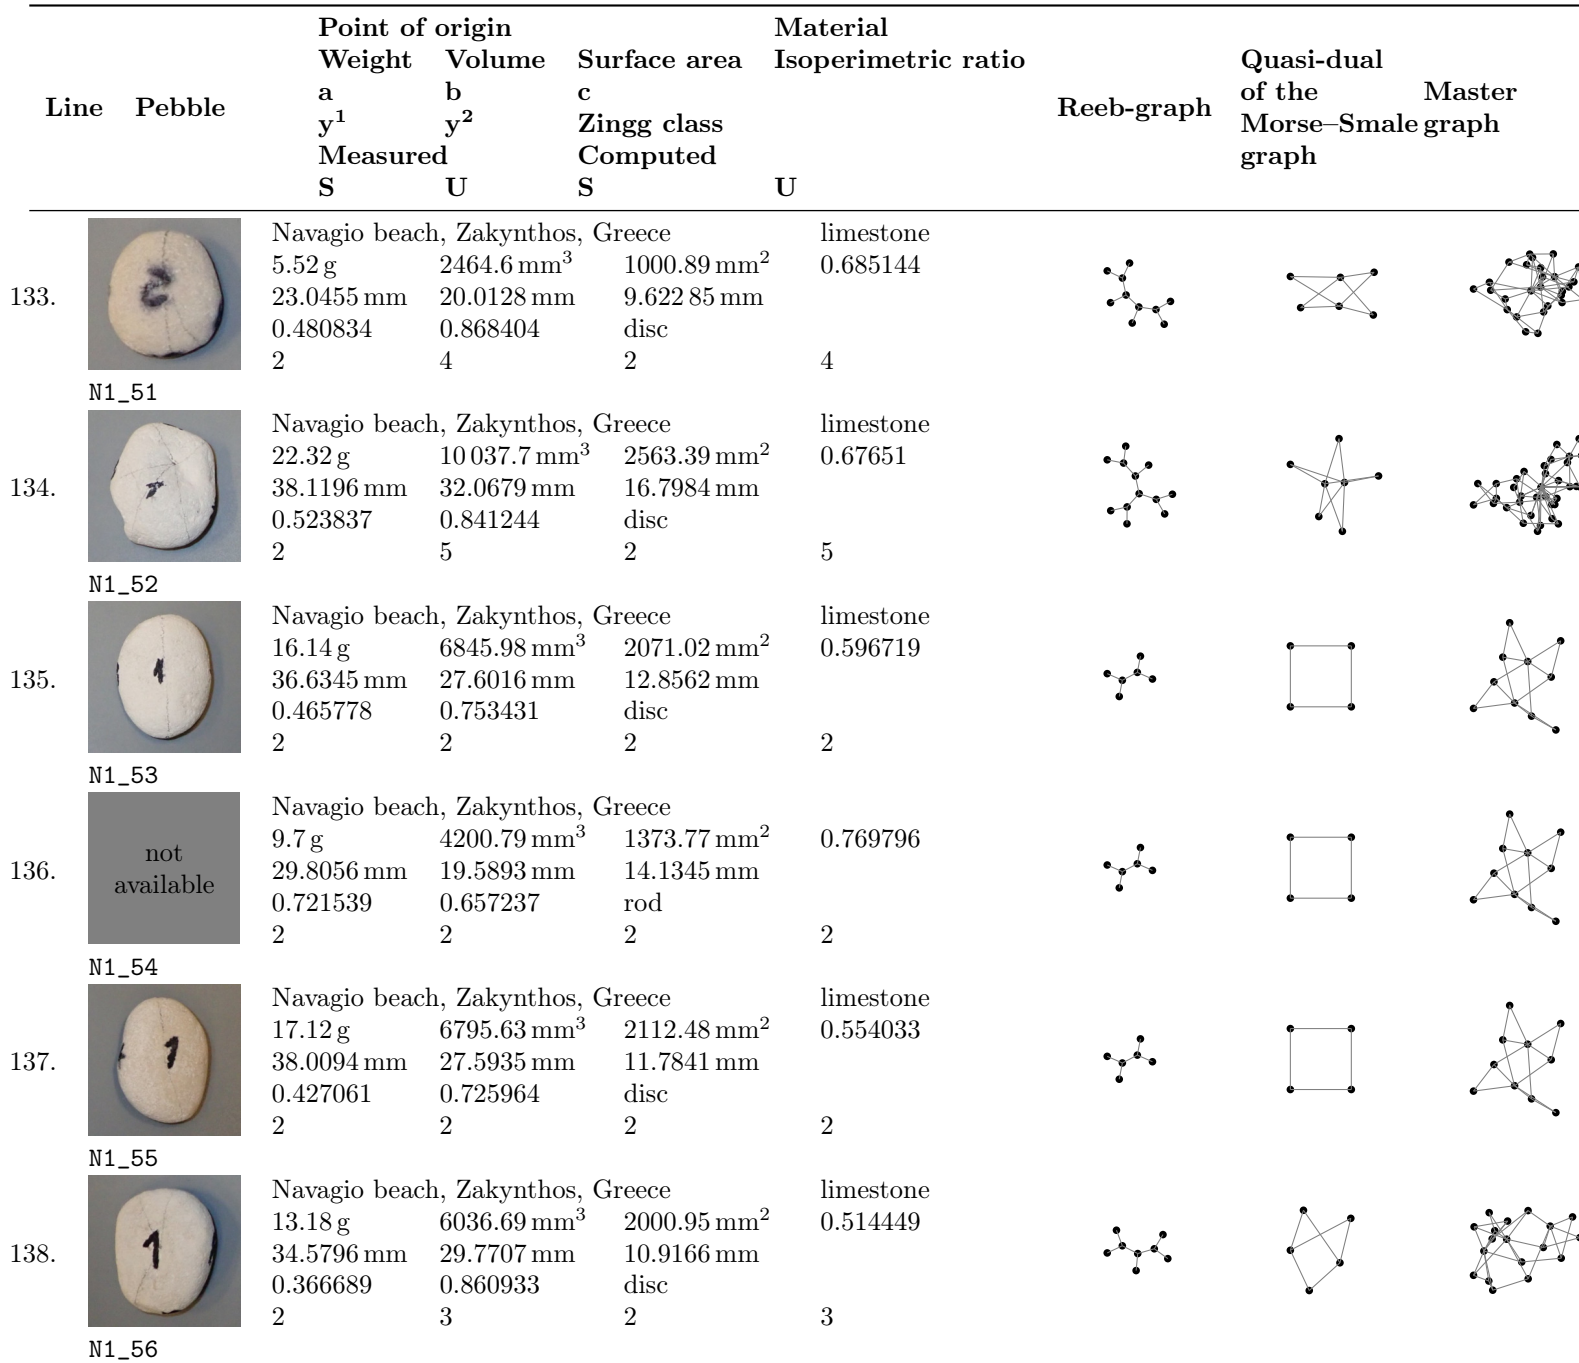   |
|      |                                                                                     | 22.32 g                          | 10 037.7 mm <sup>3</sup> | 2563.39 mm <sup>2</sup>      |                       |                                                                                       |                                                                                       |                                                                                       |
|      |                                                                                     | 38.1196 mm                       | 32.0679 mm               | 16.7984 mm                   |                       |                                                                                       |                                                                                       |                                                                                       |
|      |                                                                                     | 0.523837                         | 0.841244                 | disc                         |                       |                                                                                       |                                                                                       |                                                                                       |
|      | N1_52                                                                               | 2                                | 5                        | 2                            | 5                     |                                                                                       |                                                                                       |                                                                                       |
| 135. | 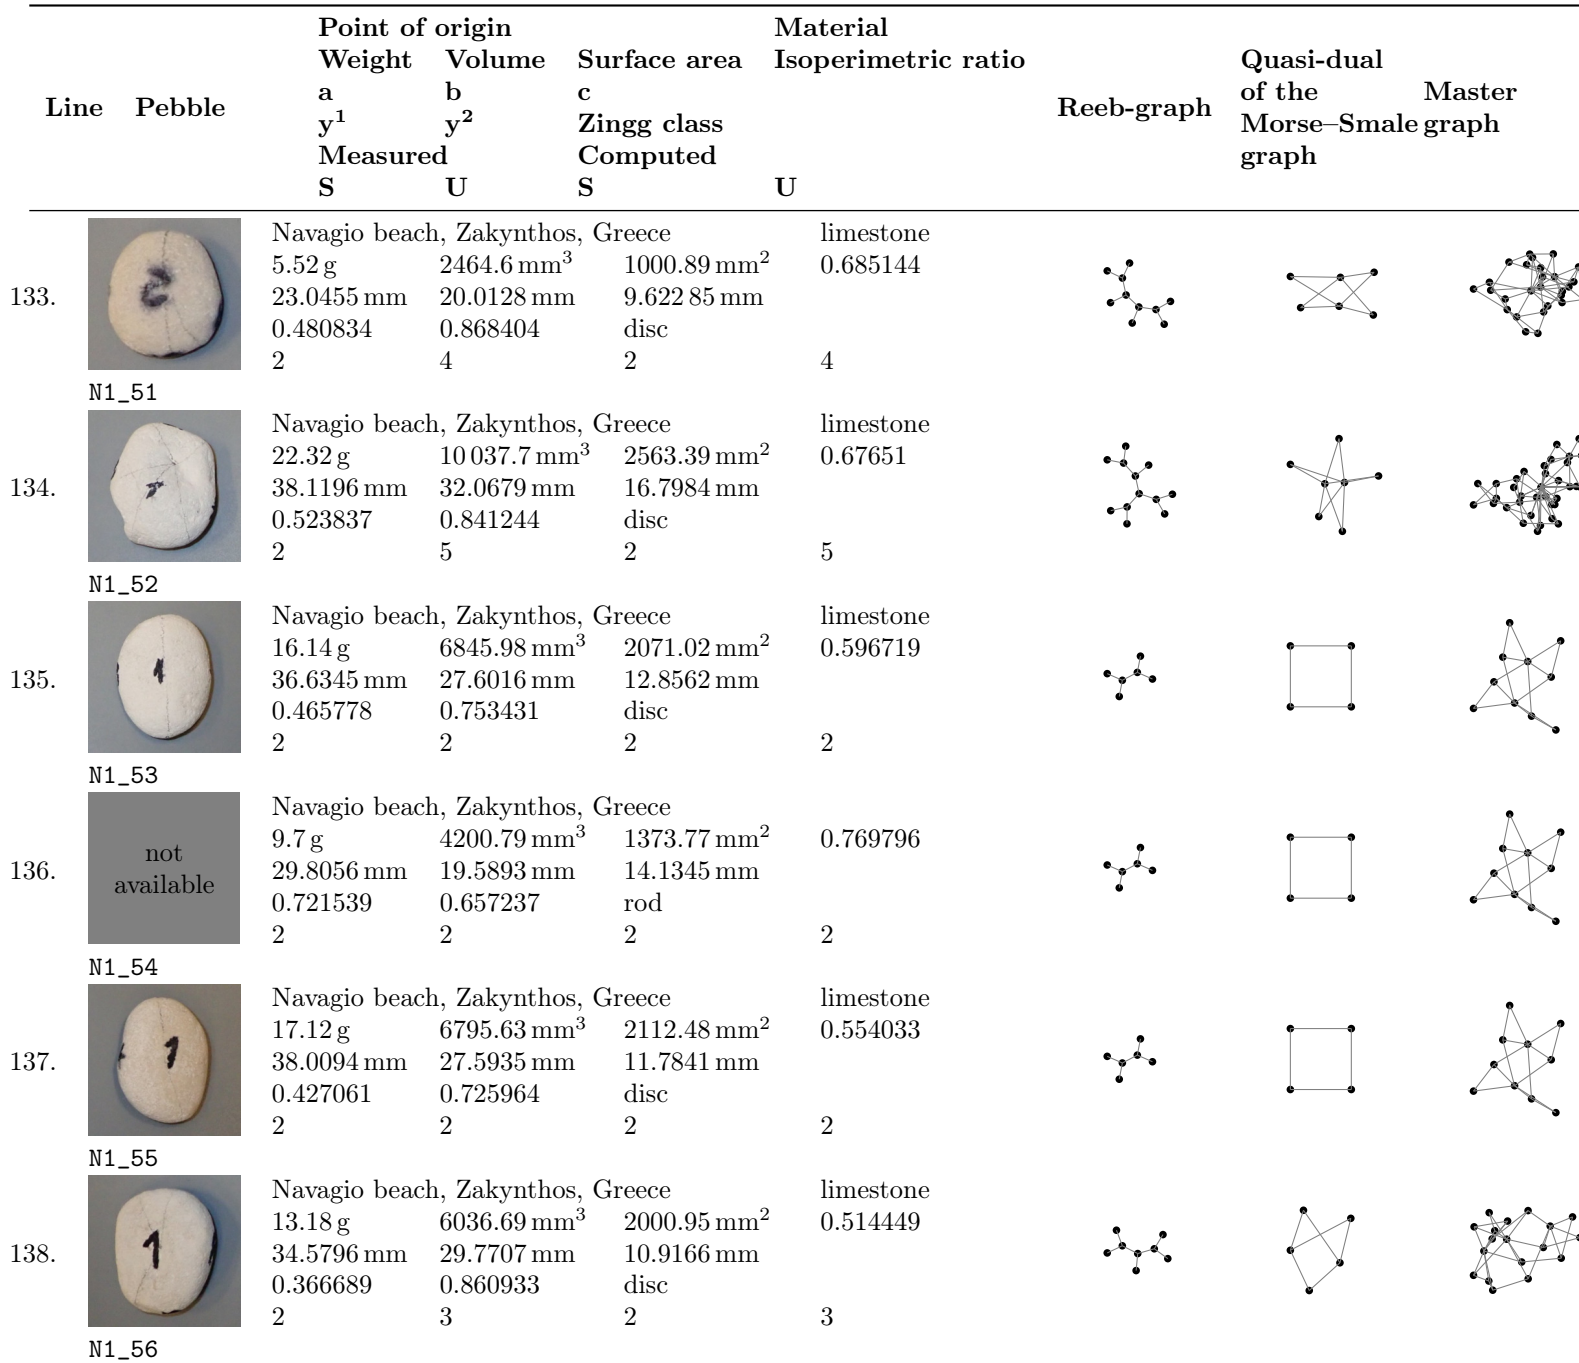   | Navagio beach, Zakynthos, Greece |                          |                              | limestone<br>0.596719 | 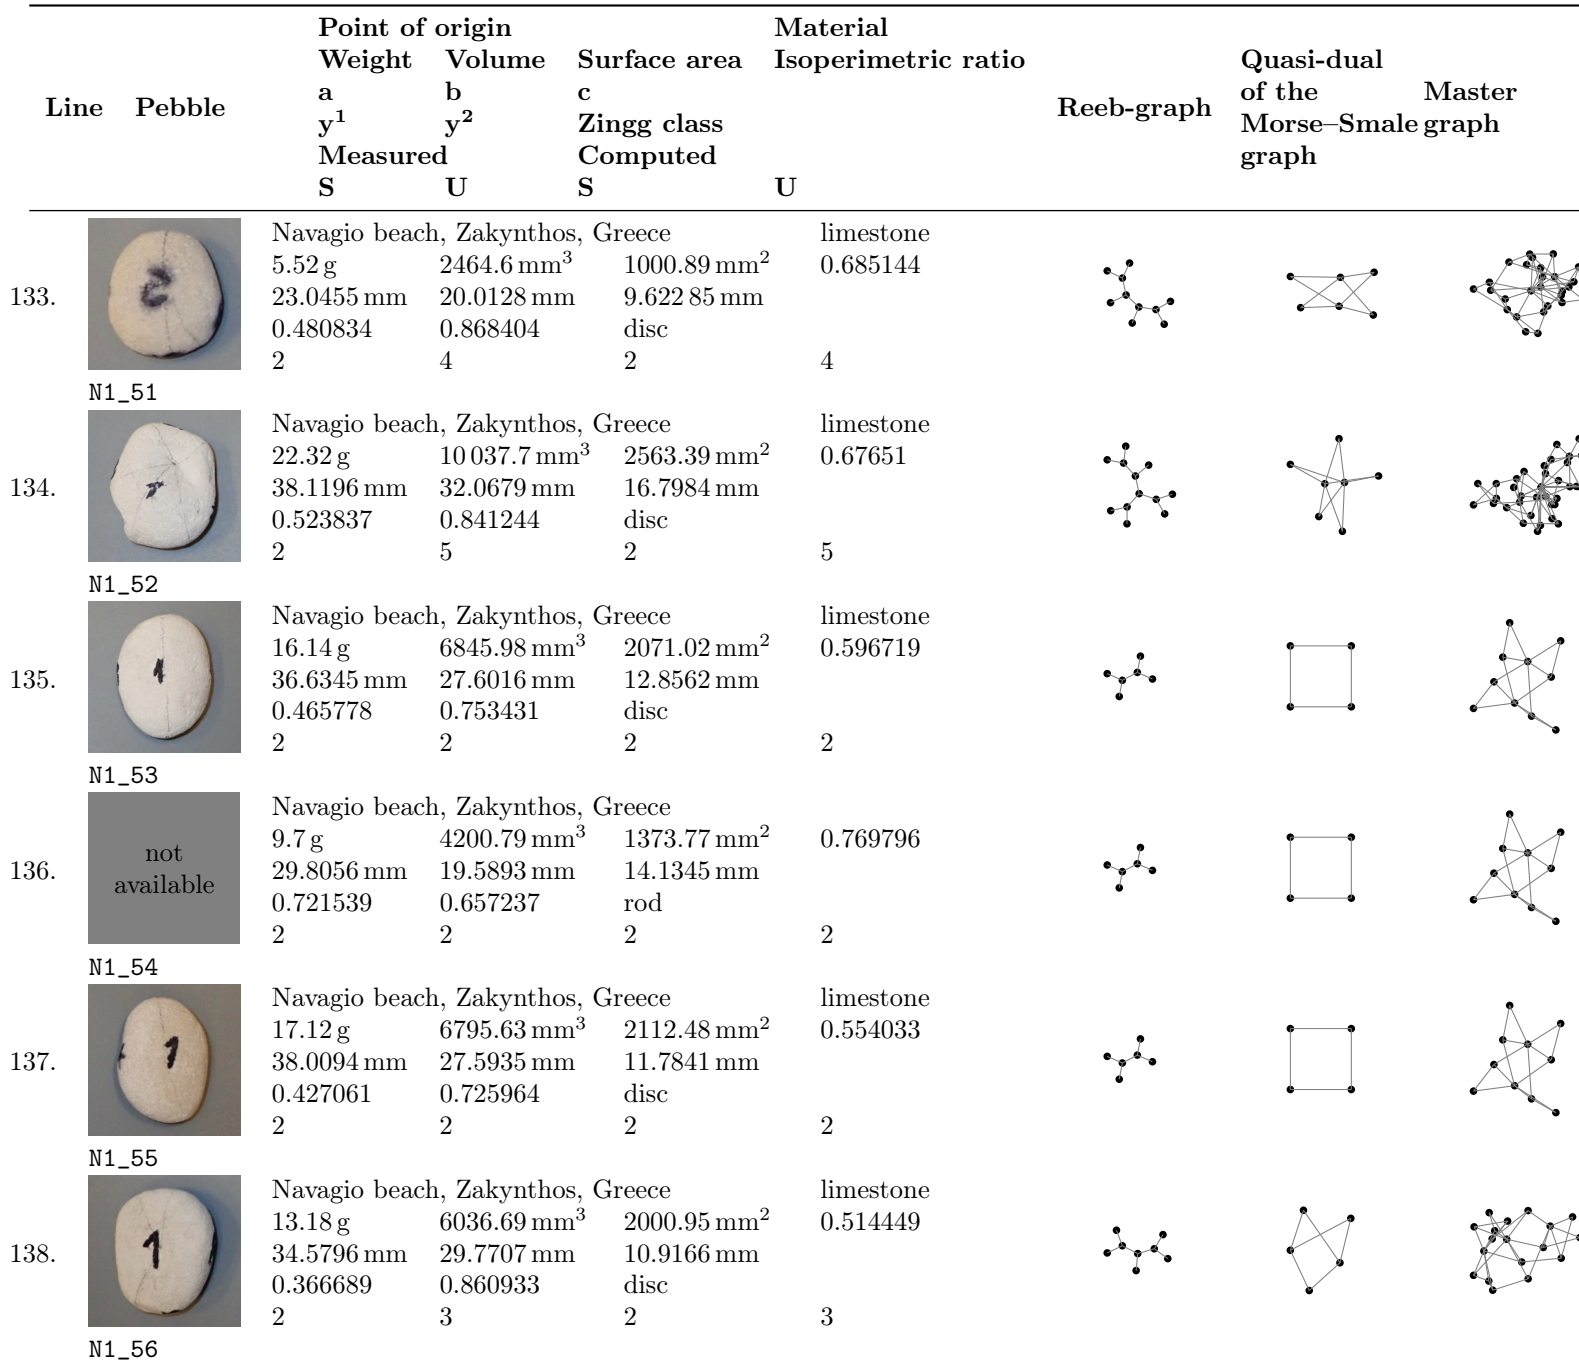   | 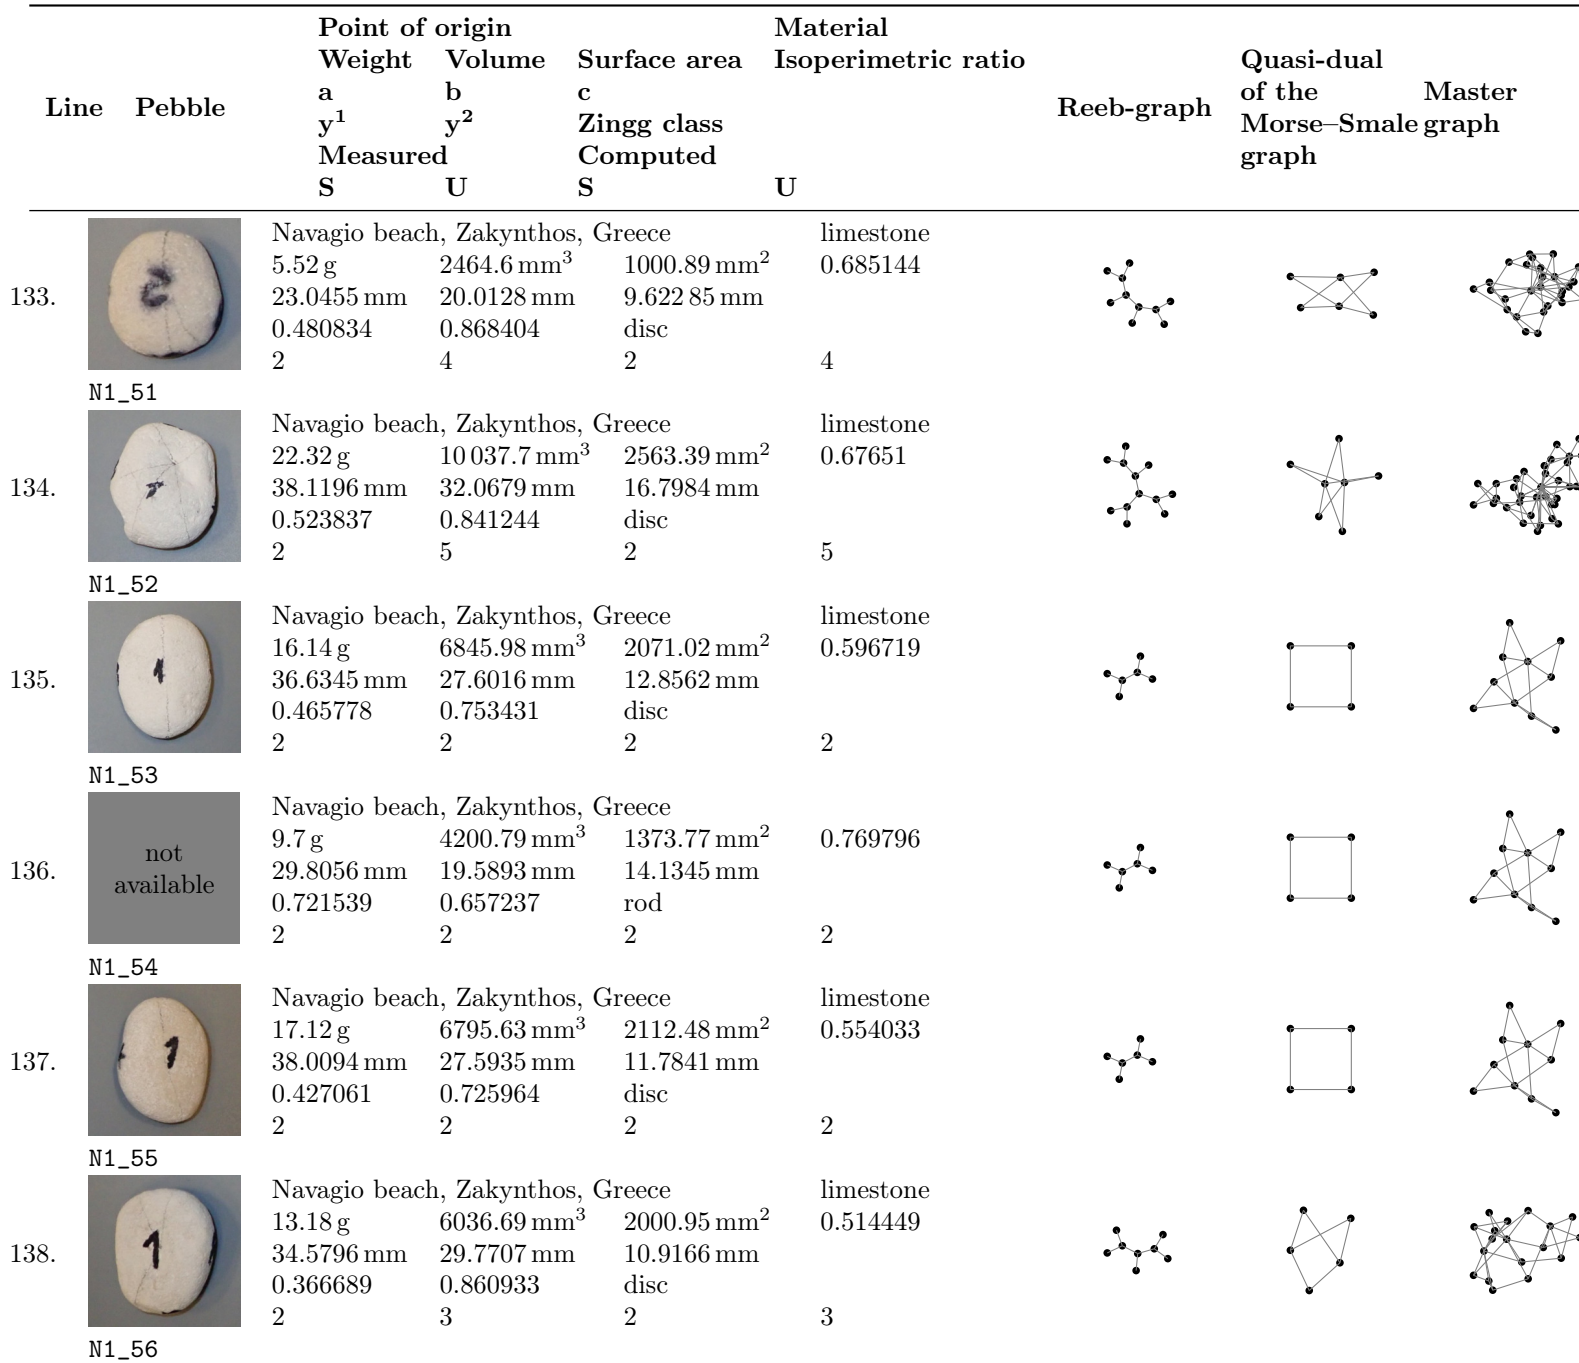   | 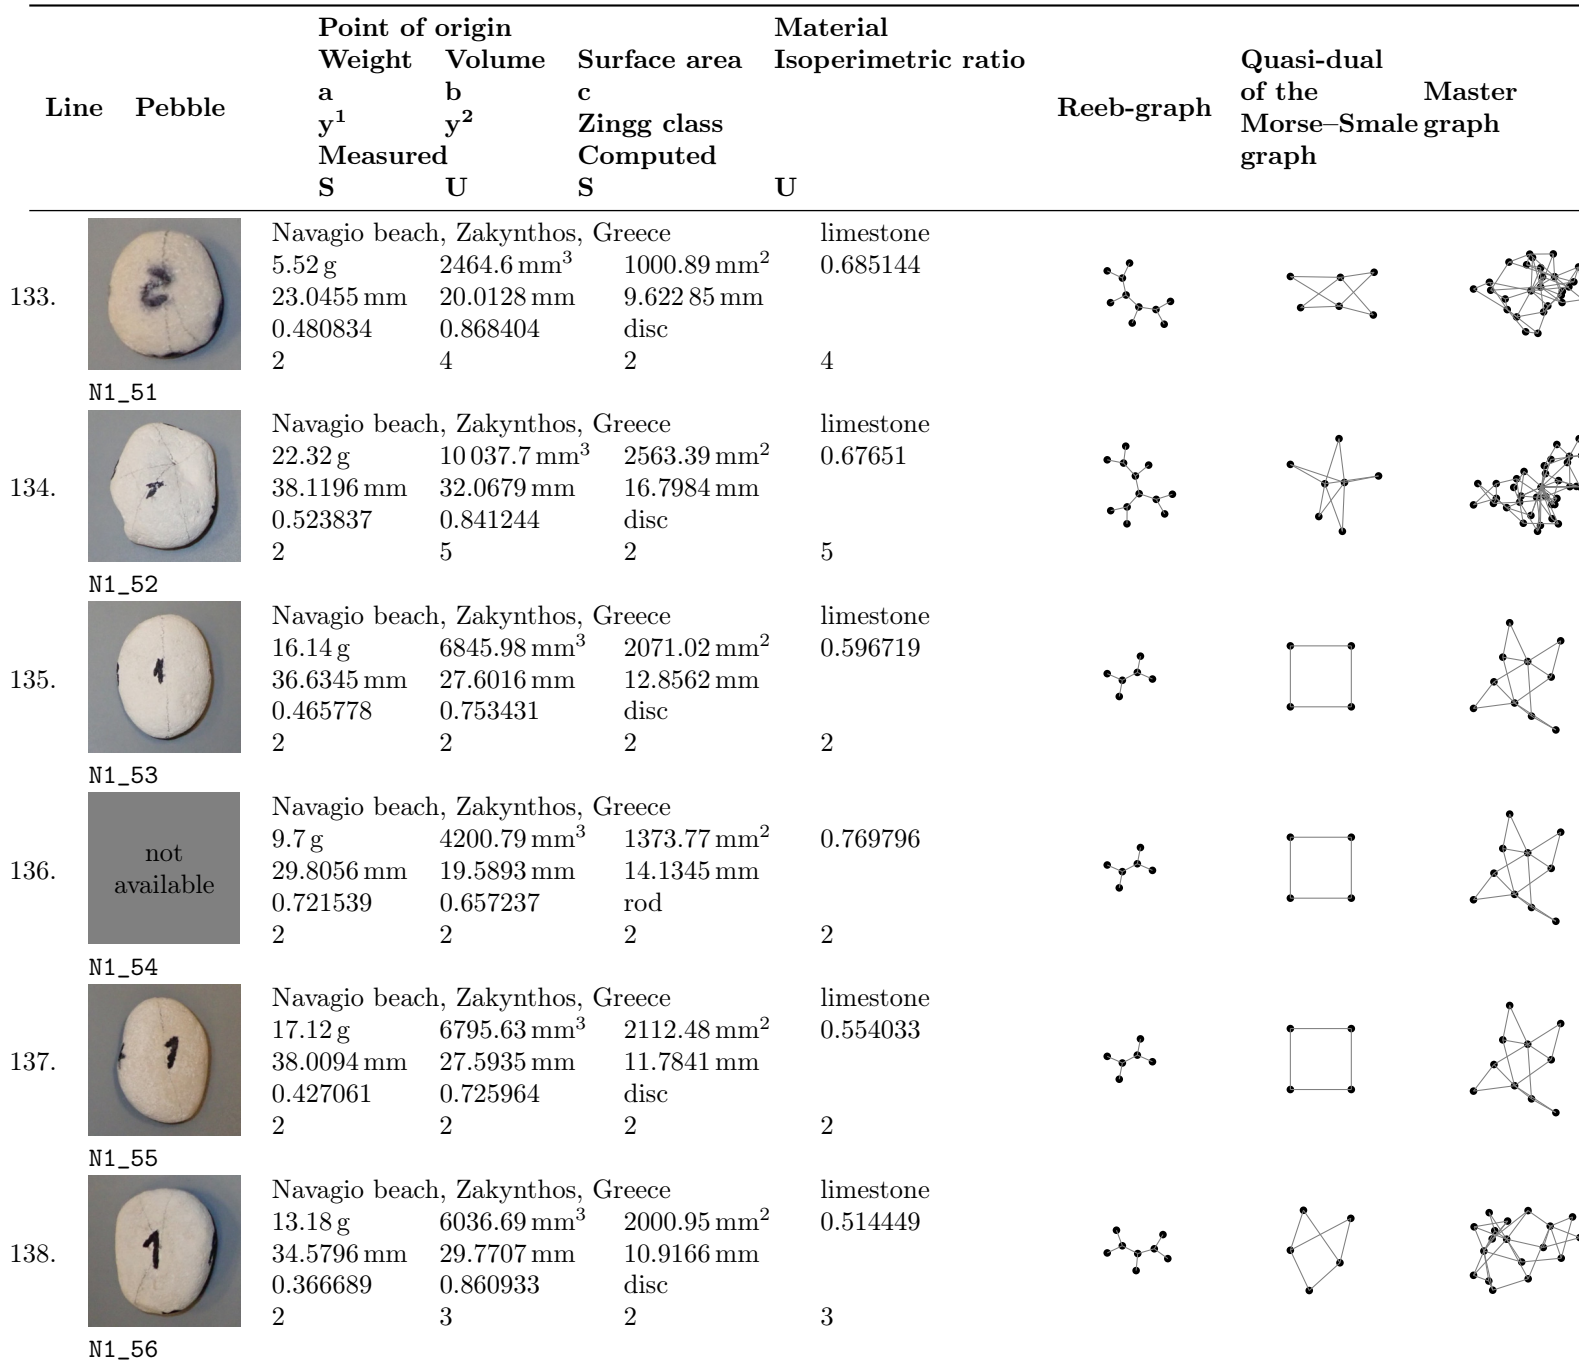   |
|      |                                                                                     | 16.14 g                          | 6845.98 mm <sup>3</sup>  | 2071.02 mm <sup>2</sup>      |                       |                                                                                       |                                                                                       |                                                                                       |
|      |                                                                                     | 36.6345 mm                       | 27.6016 mm               | 12.8562 mm                   |                       |                                                                                       |                                                                                       |                                                                                       |
|      |                                                                                     | 0.465778                         | 0.753431                 | disc                         |                       |                                                                                       |                                                                                       |                                                                                       |
|      | N1_53                                                                               | 2                                | 2                        | 2                            | 2                     |                                                                                       |                                                                                       |                                                                                       |
| 136. | 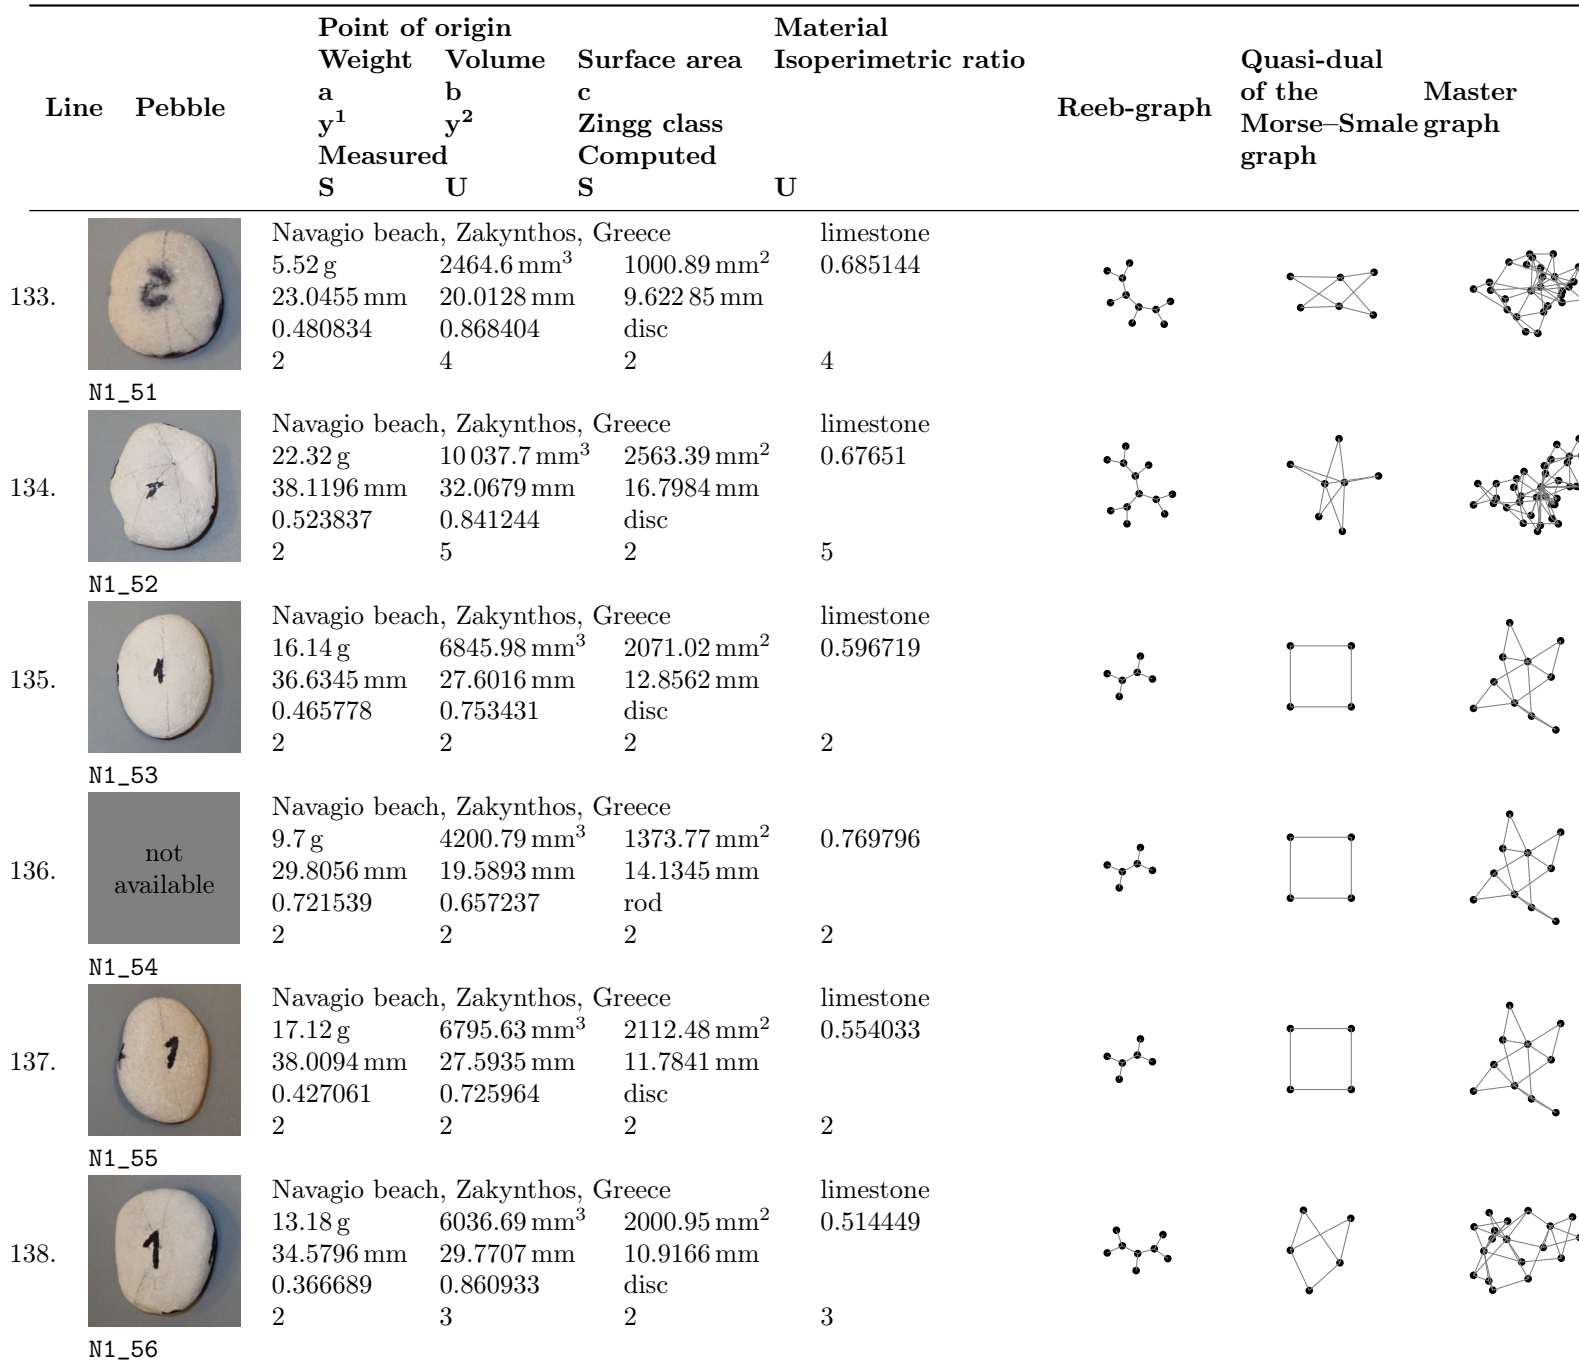  | Navagio beach, Zakynthos, Greece |                          |                              | limestone<br>0.769796 | 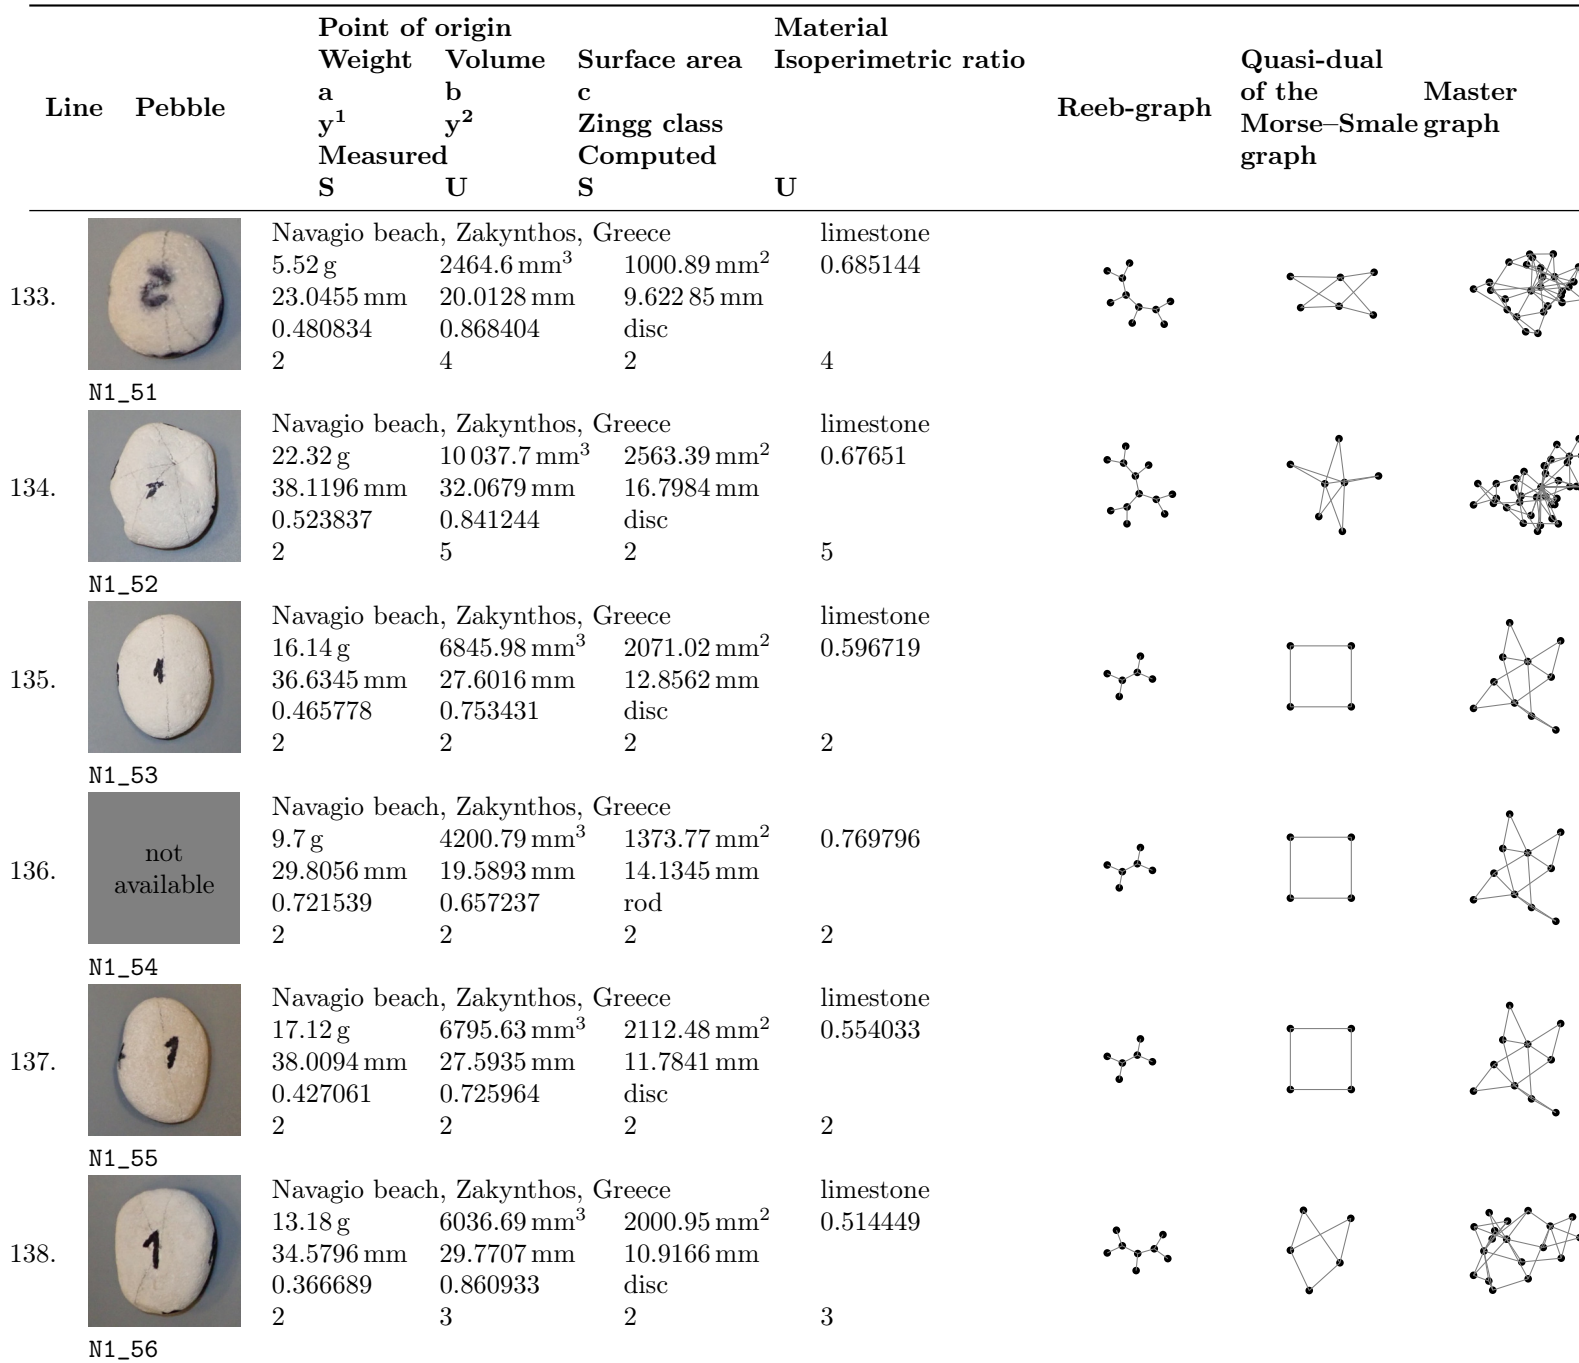  | 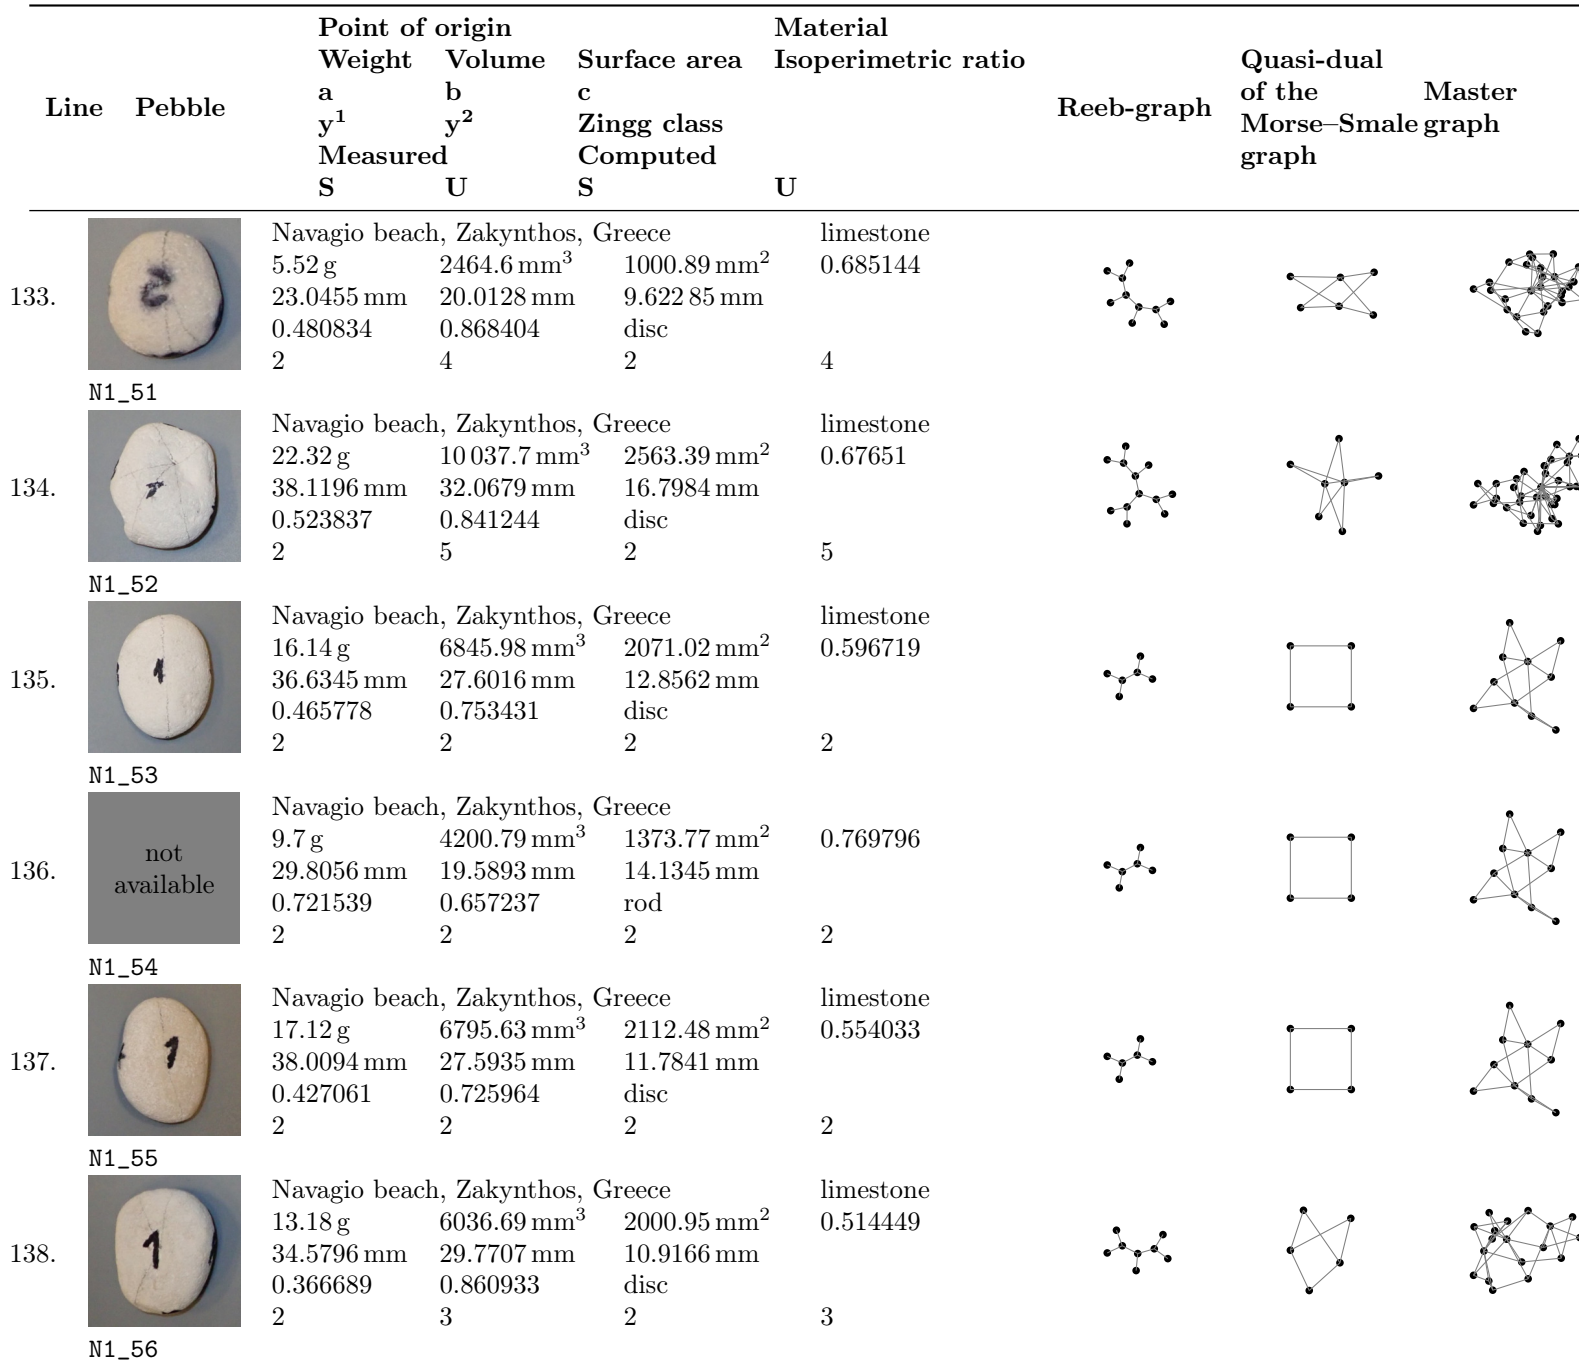  | 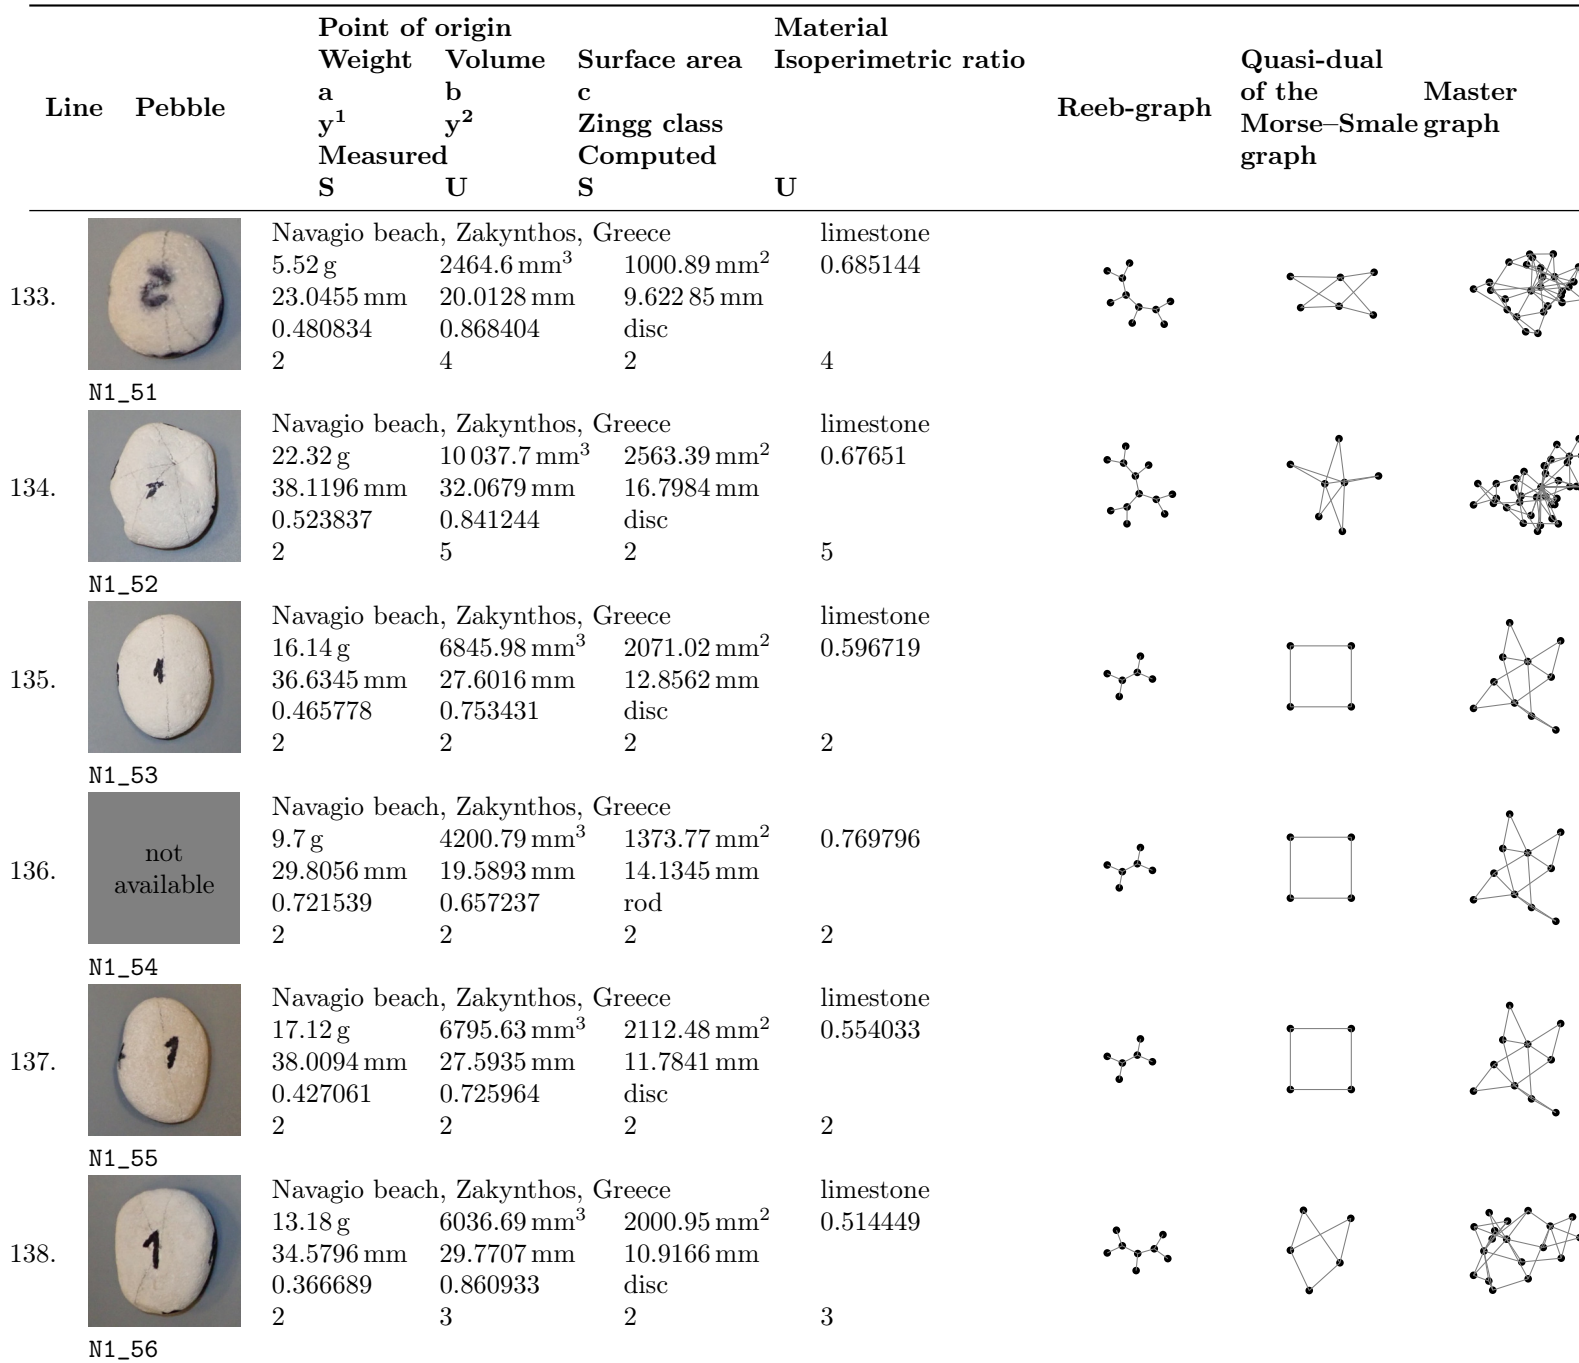  |
|      |                                                                                     | 9.7 g                            | 4200.79 mm <sup>3</sup>  | 1373.77 mm <sup>2</sup>      |                       |                                                                                       |                                                                                       |                                                                                       |
|      |                                                                                     | 29.8056 mm                       | 19.5893 mm               | 14.1345 mm                   |                       |                                                                                       |                                                                                       |                                                                                       |
|      |                                                                                     | 0.721539                         | 0.657237                 | rod                          |                       |                                                                                       |                                                                                       |                                                                                       |
|      | N1_54                                                                               | 2                                | 2                        | 2                            | 2                     |                                                                                       |                                                                                       |                                                                                       |
| 137. | 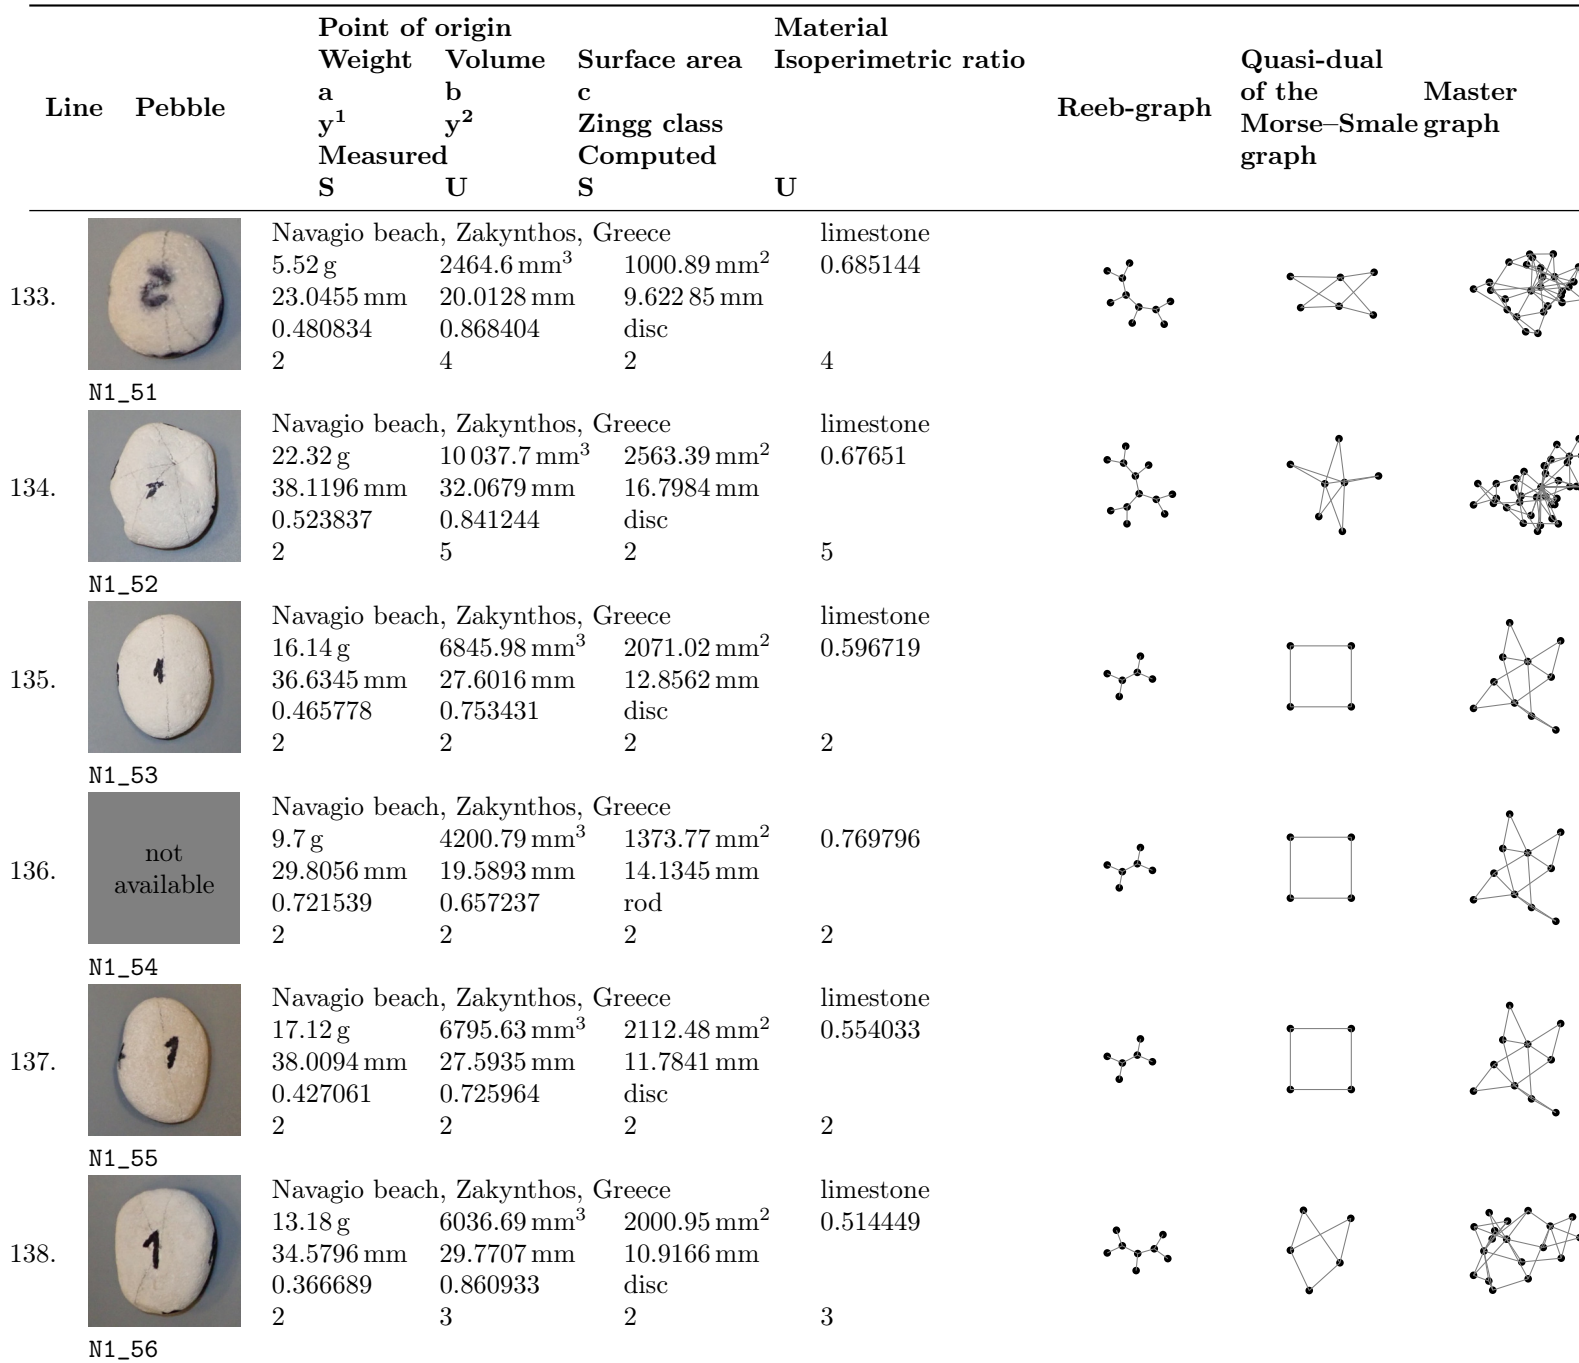 | Navagio beach, Zakynthos, Greece |                          |                              | limestone<br>0.554033 | 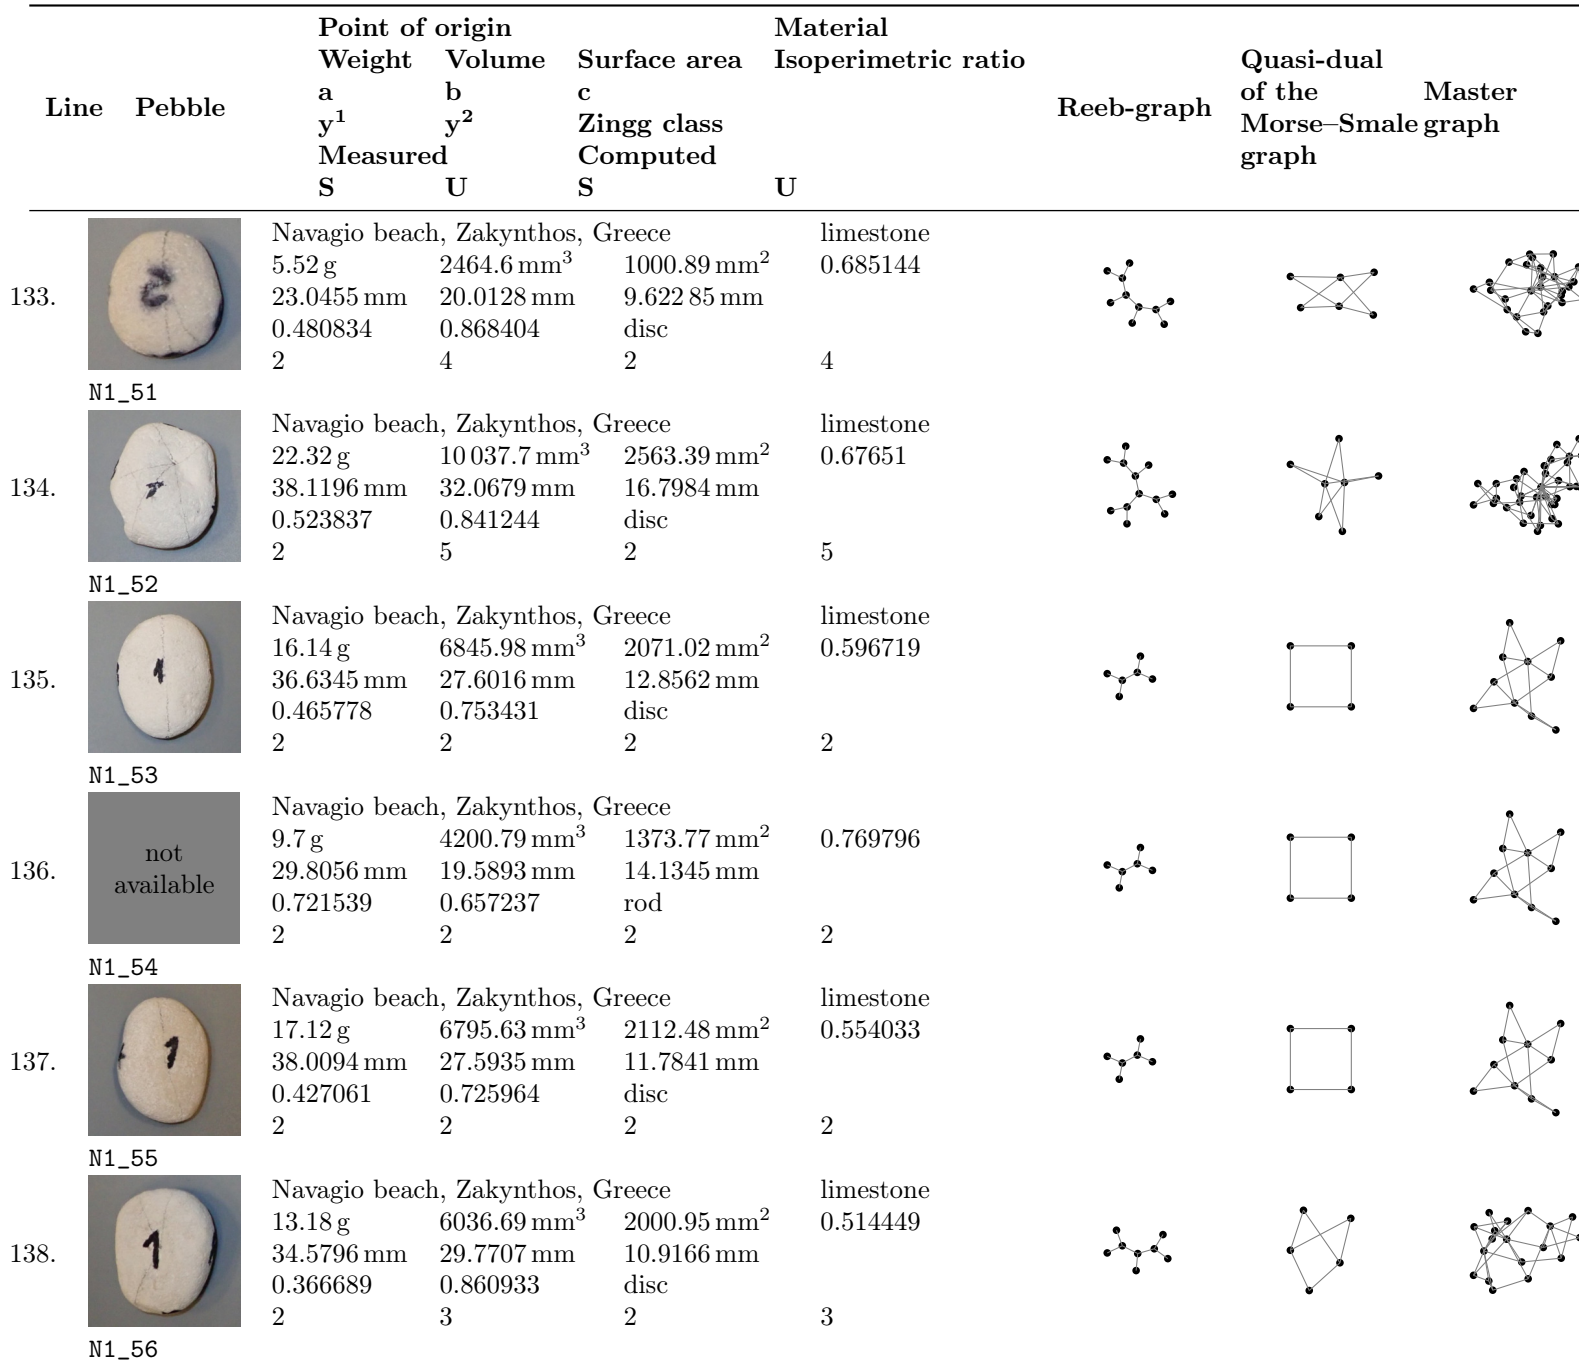 | 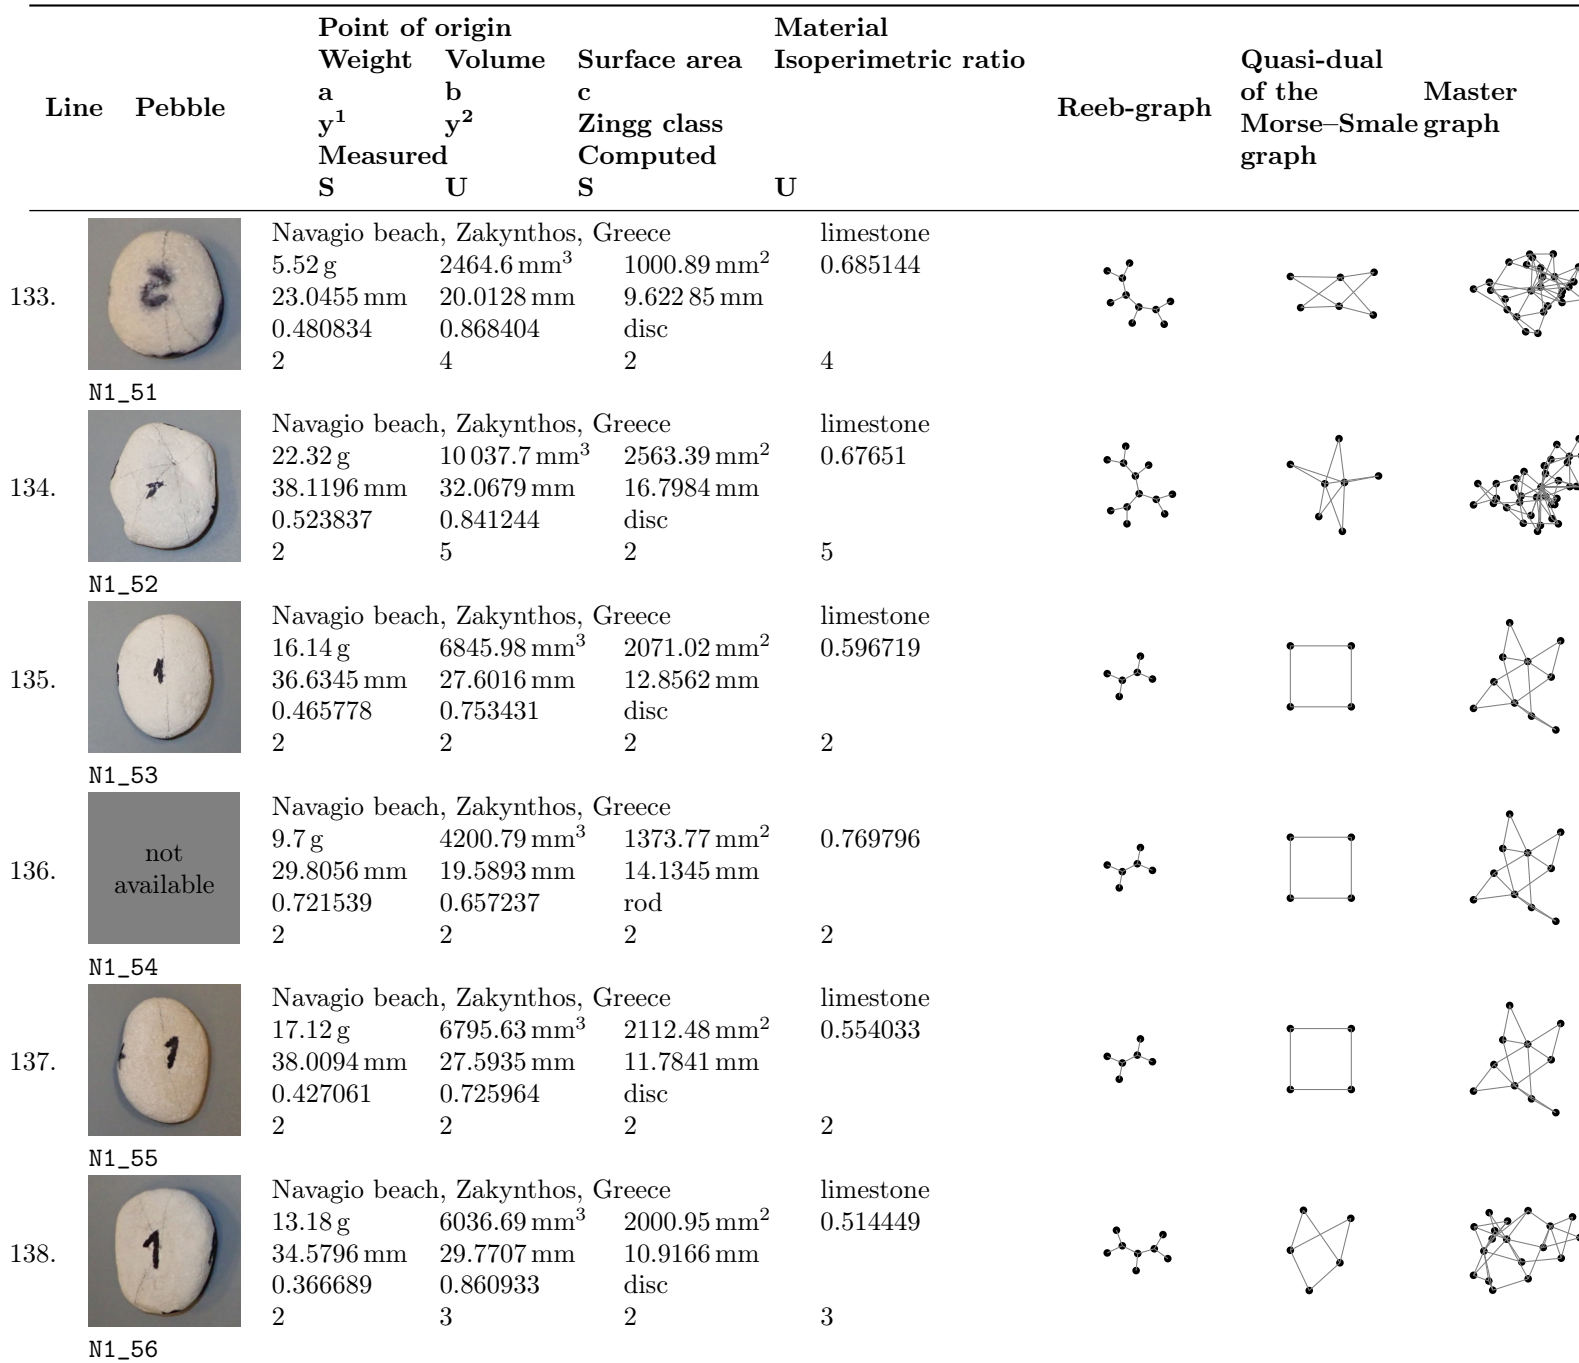 | 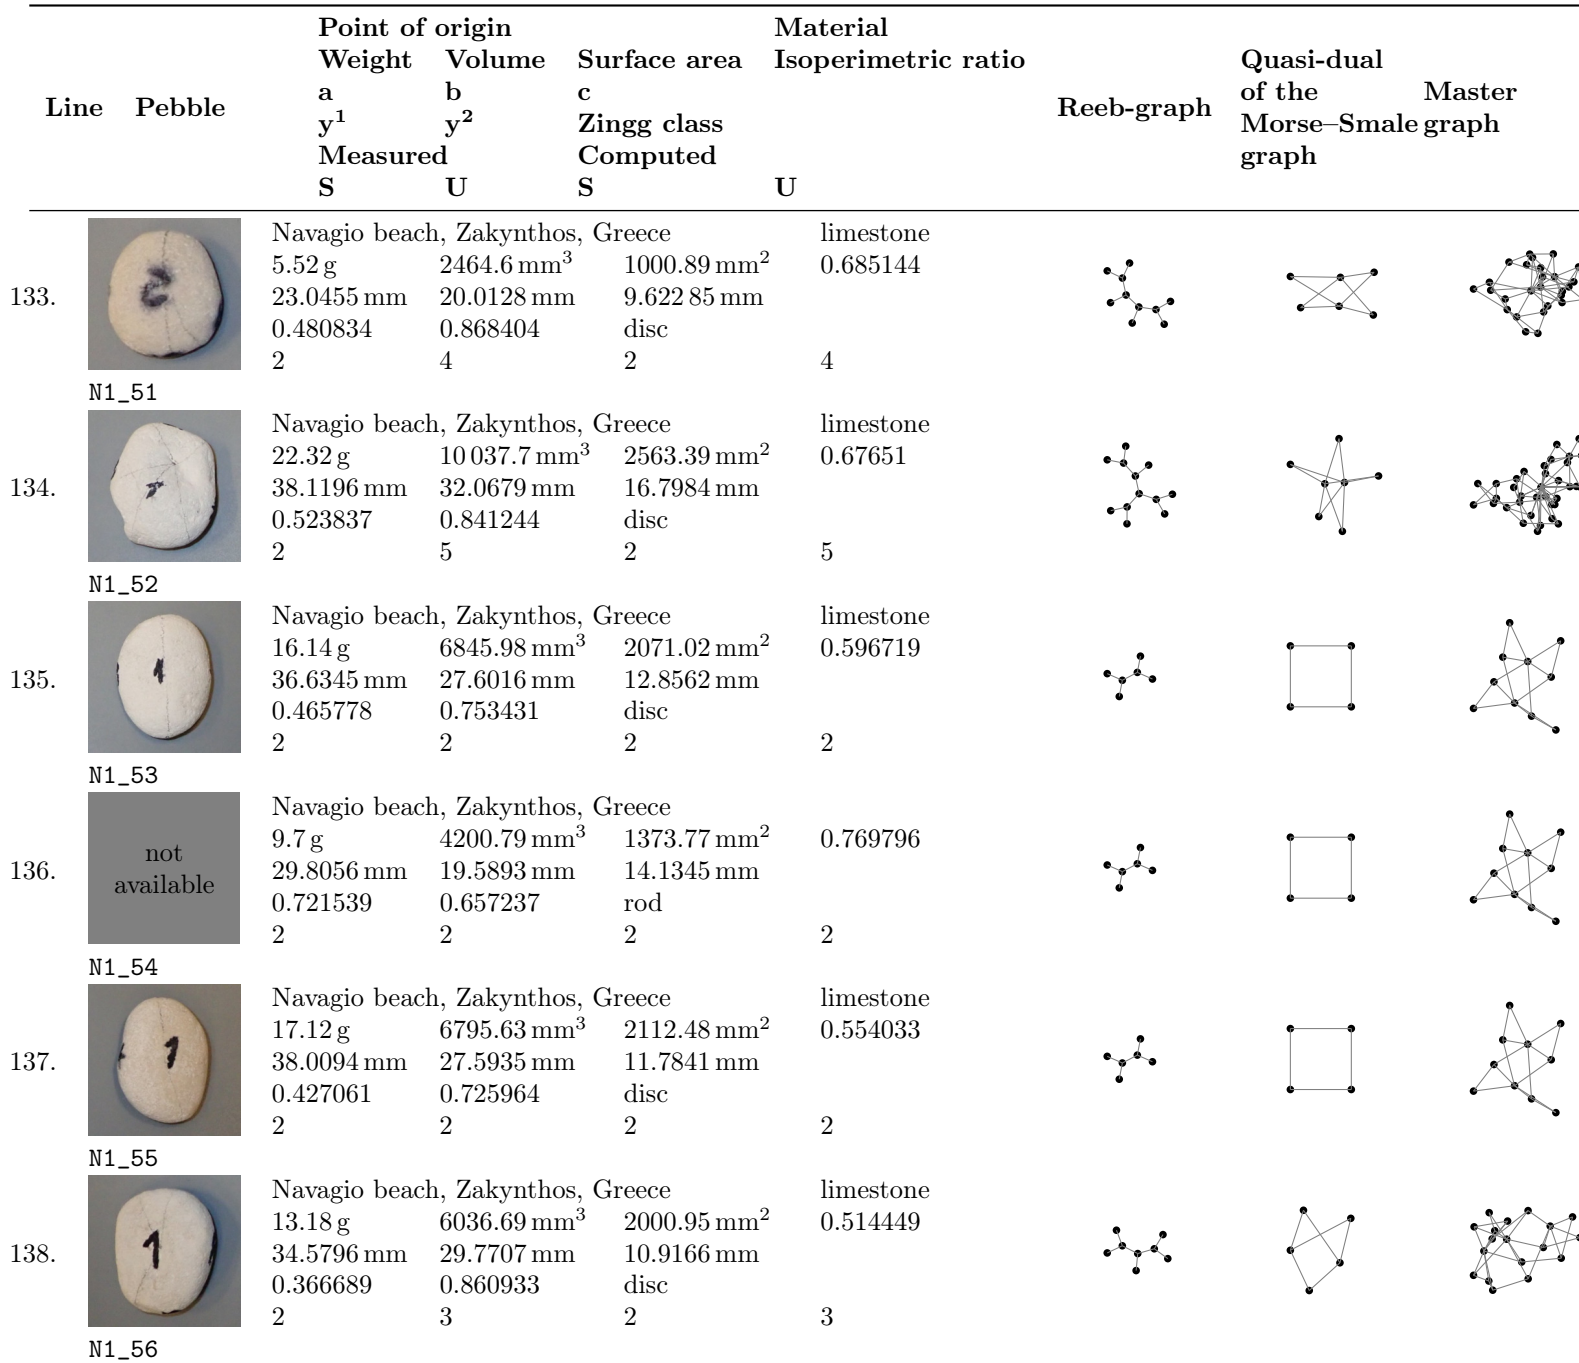 |
|      |                                                                                     | 17.12 g                          | 6795.63 mm <sup>3</sup>  | 2112.48 mm <sup>2</sup>      |                       |                                                                                       |                                                                                       |                                                                                       |
|      |                                                                                     | 38.0094 mm                       | 27.5935 mm               | 11.7841 mm                   |                       |                                                                                       |                                                                                       |                                                                                       |
|      |                                                                                     | 0.427061                         | 0.725964                 | disc                         |                       |                                                                                       |                                                                                       |                                                                                       |
|      | N1_55                                                                               | 2                                | 2                        | 2                            | 2                     |                                                                                       |                                                                                       |                                                                                       |
| 138. | 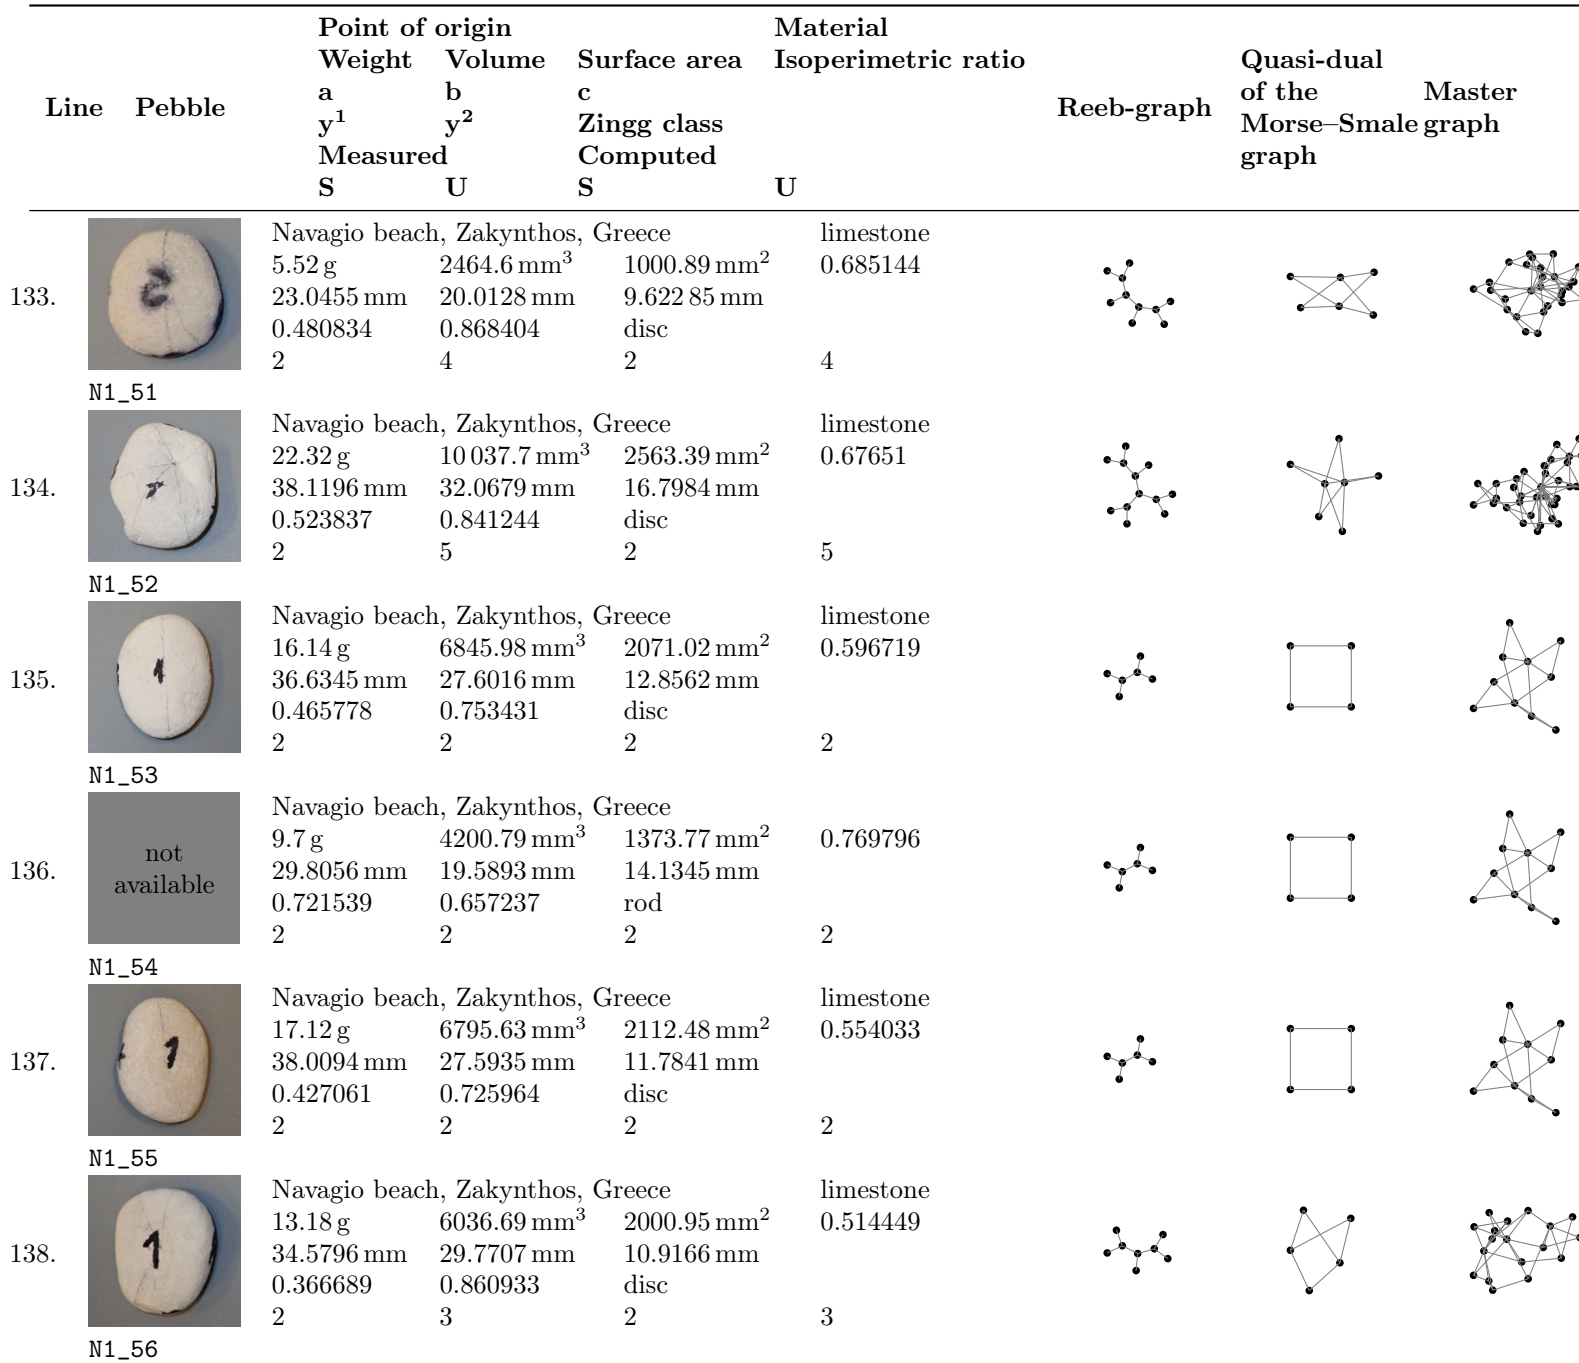 | Navagio beach, Zakynthos, Greece |                          |                              | limestone<br>0.514449 | 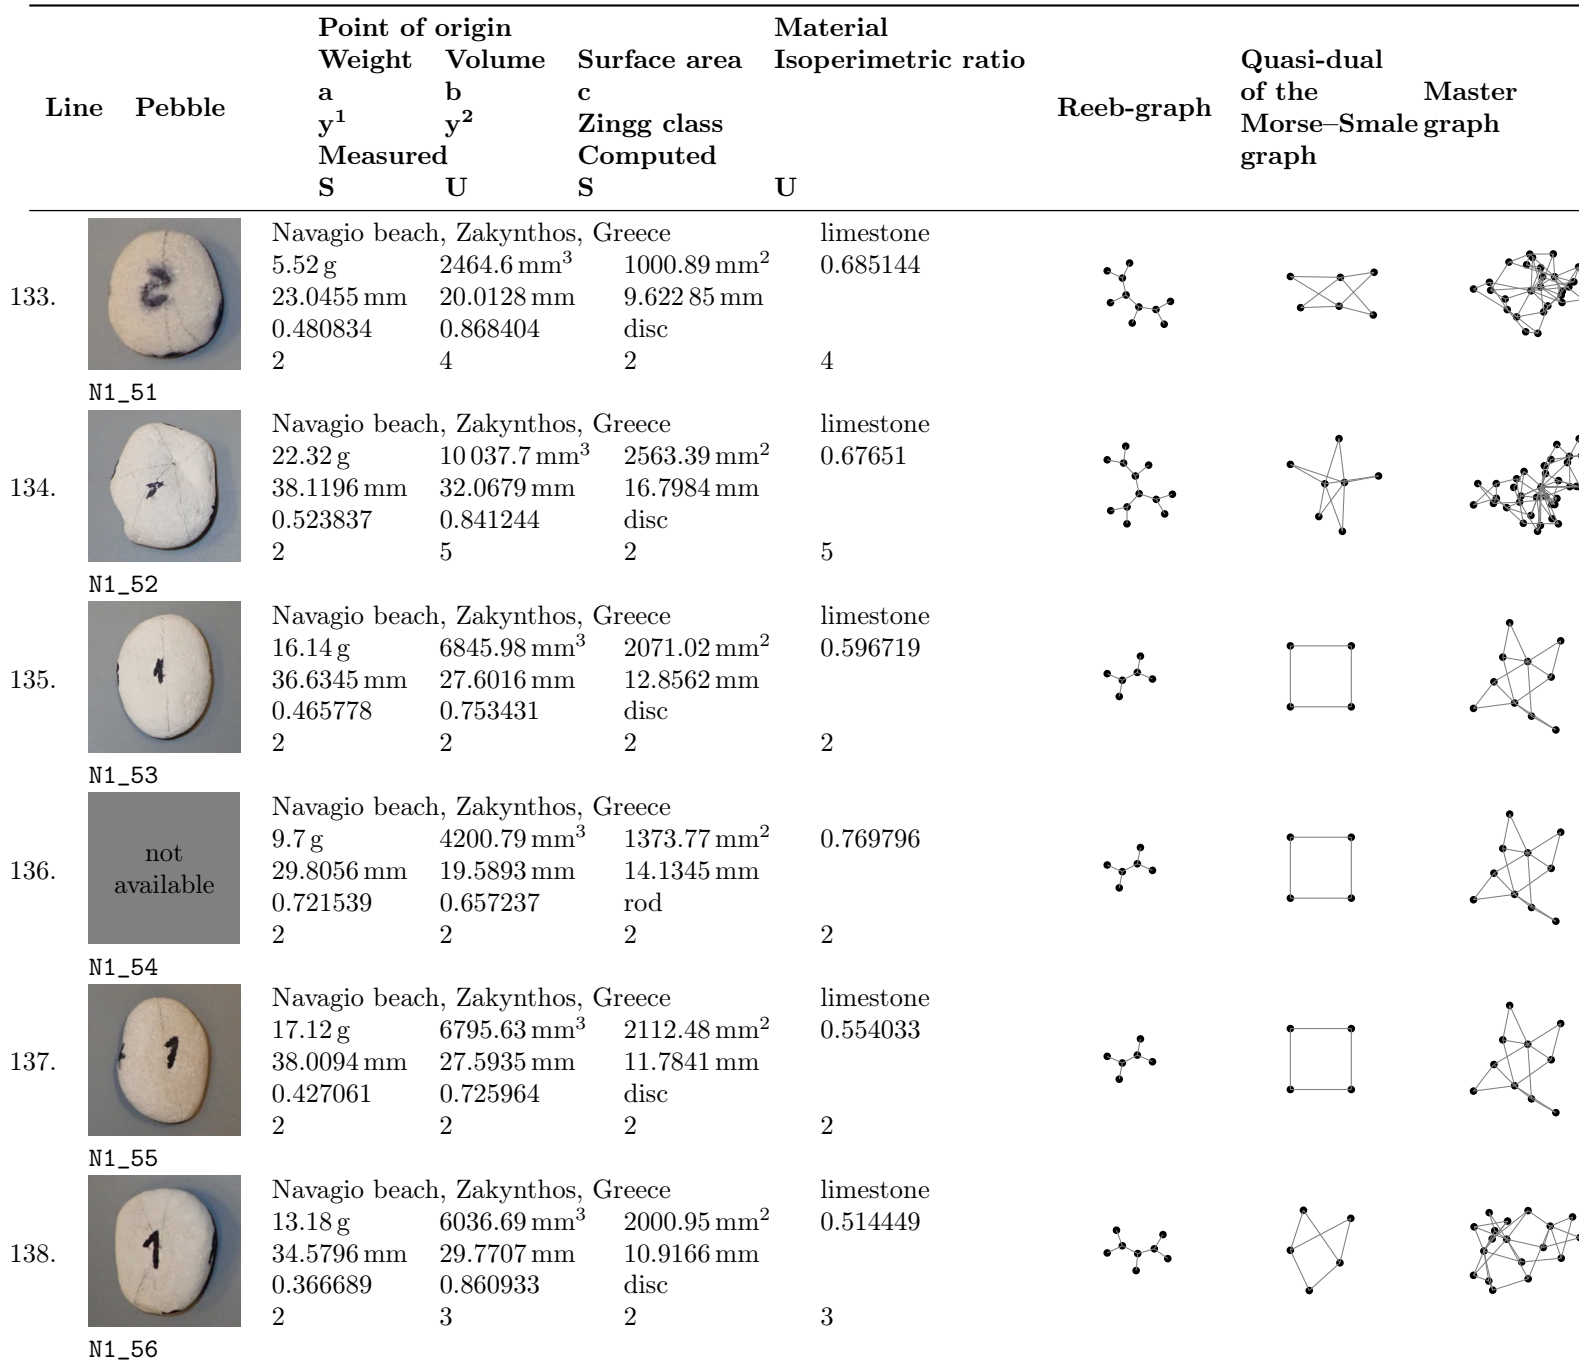 | 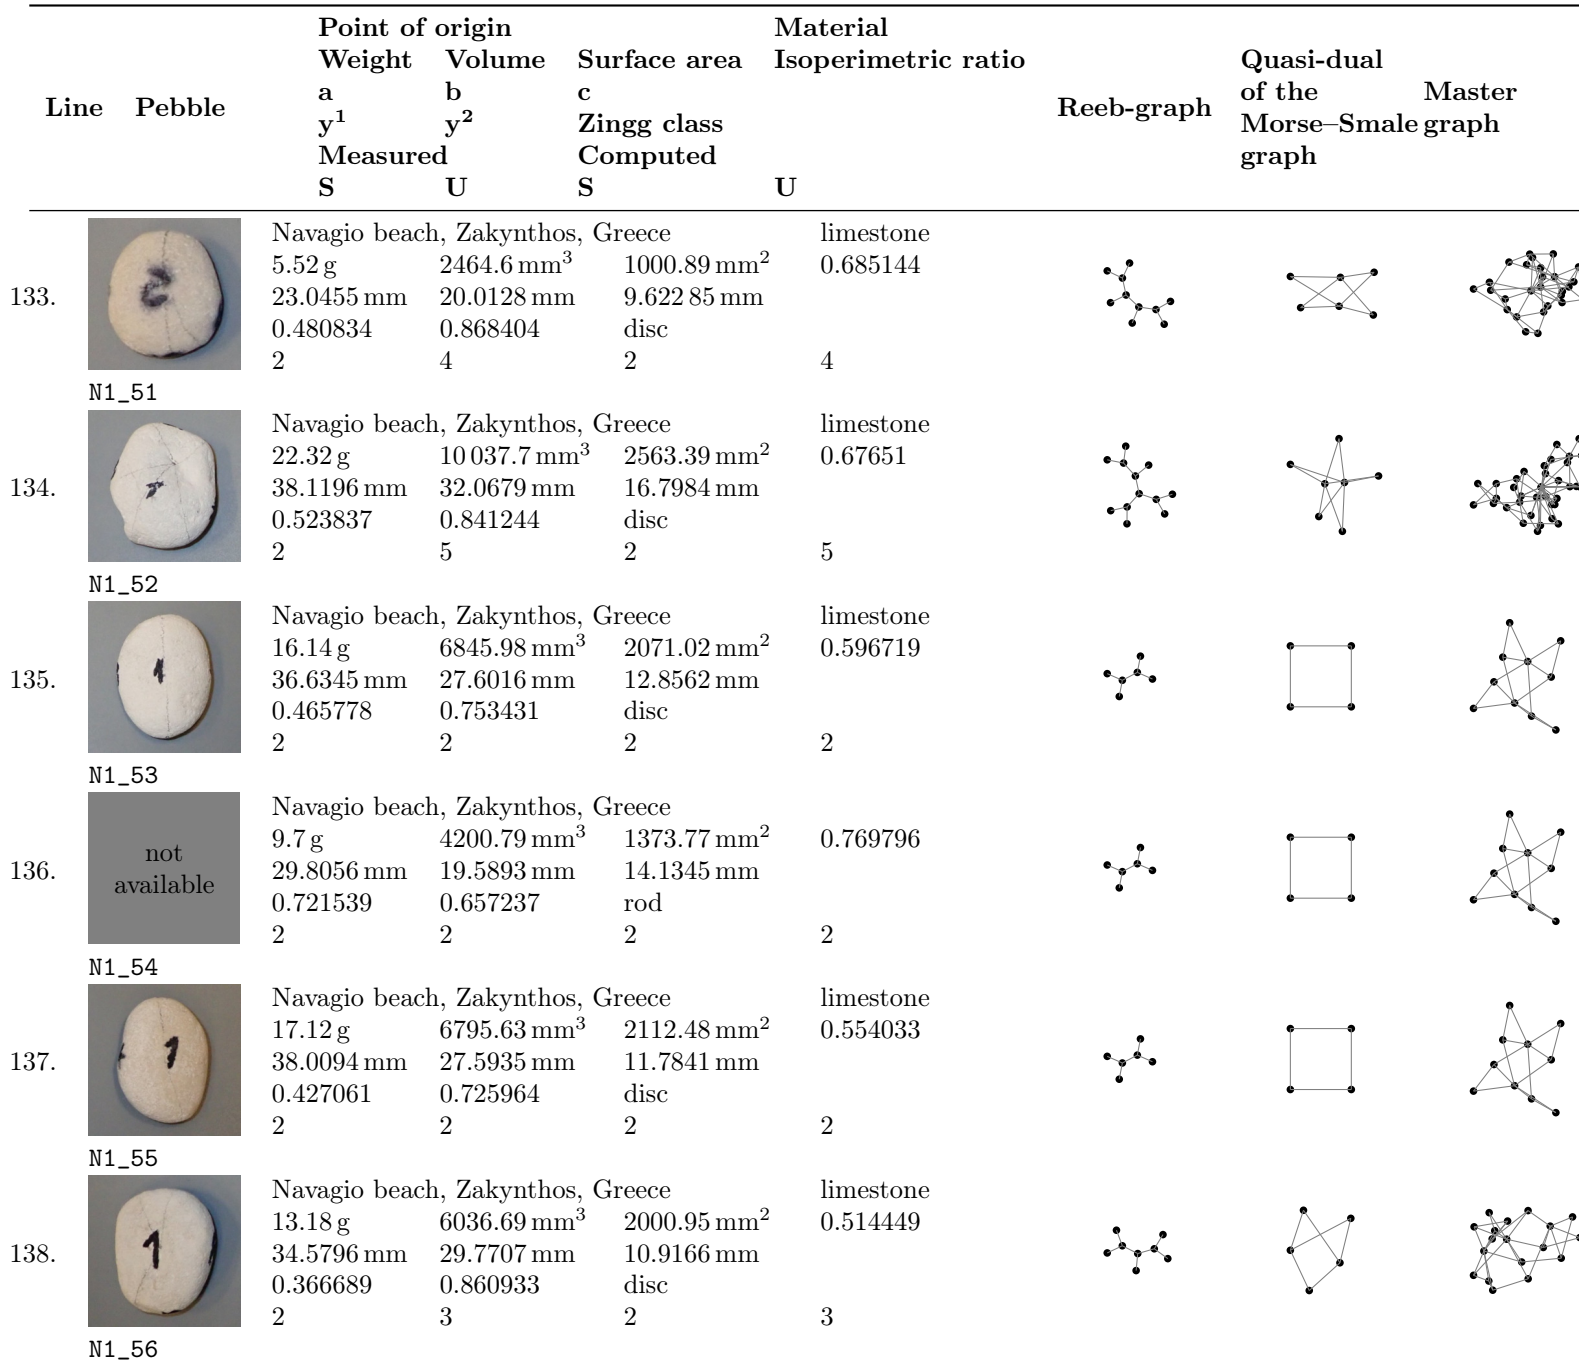 | 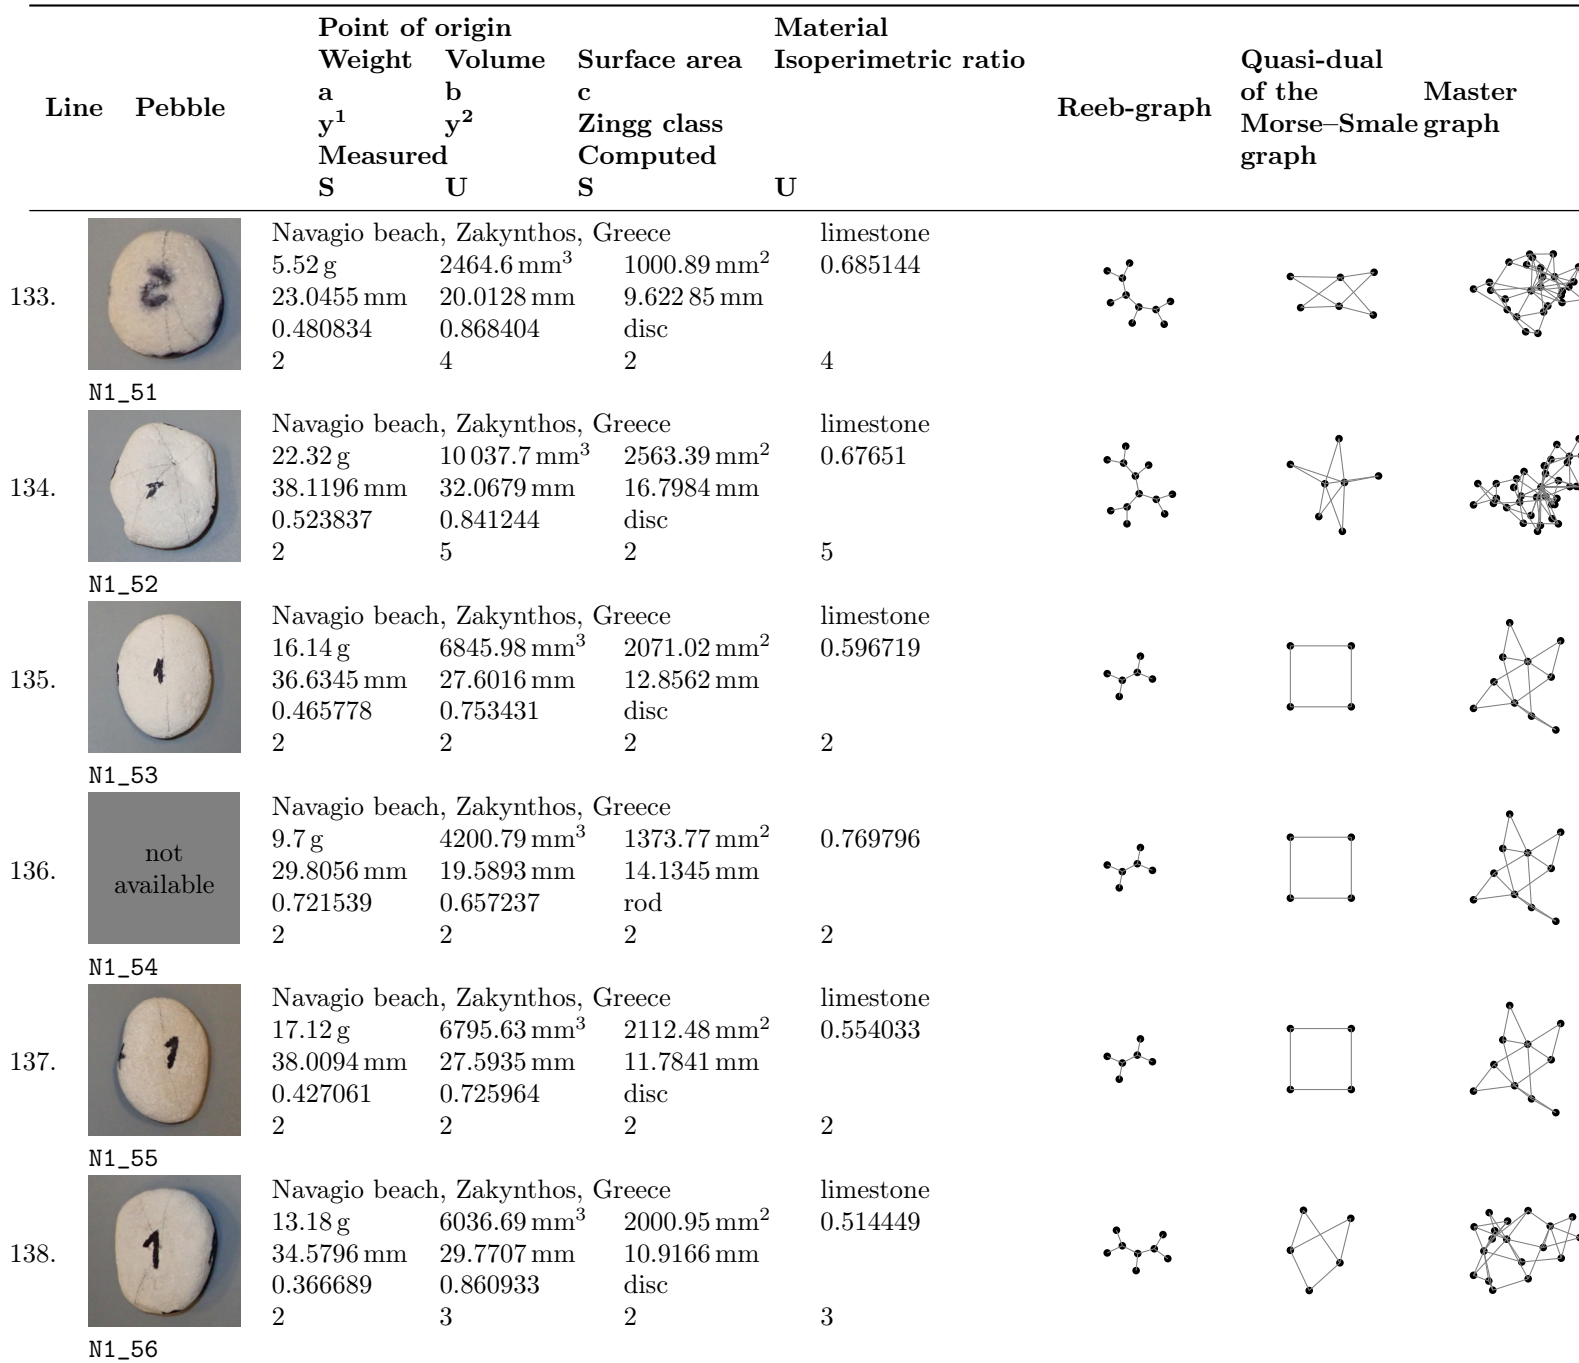 |
|      |                                                                                     | 13.18 g                          | 6036.69 mm <sup>3</sup>  | 2000.95 mm <sup>2</sup>      |                       |                                                                                       |                                                                                       |                                                                                       |
|      |                                                                                     | 34.5796 mm                       | 29.7707 mm               | 10.9166 mm                   |                       |                                                                                       |                                                                                       |                                                                                       |
|      |                                                                                     | 0.366689                         | 0.860933                 | disc                         |                       |                                                                                       |                                                                                       |                                                                                       |
|      | N1_56                                                                               | 2                                | 3                        | 2                            | 3                     |                                                                                       |                                                                                       |                                                                                       |

| Line | Pebble                        | Point of origin                  |                         |                              | Material<br>Isoperimetric ratio<br>U | Reeb-graph                                                                            | Quasi-dual<br>of the<br>Morse–Smale<br>graph                                          | Master<br>graph                                                                       |
|------|-------------------------------|----------------------------------|-------------------------|------------------------------|--------------------------------------|---------------------------------------------------------------------------------------|---------------------------------------------------------------------------------------|---------------------------------------------------------------------------------------|
|      |                               | Weight                           | Volume                  | Surface area                 |                                      |                                                                                       |                                                                                       |                                                                                       |
|      |                               | a                                | b                       | c                            |                                      |                                                                                       |                                                                                       |                                                                                       |
|      |                               | y <sup>1</sup><br>Measured<br>S  | y <sup>2</sup><br>U     | Zingg class<br>Computed<br>S |                                      |                                                                                       |                                                                                       |                                                                                       |
| 139. | not<br>available<br><br>N1_57 | Navagio beach, Zakynthos, Greece |                         |                              | 0.588588<br><br><br><br>3            | 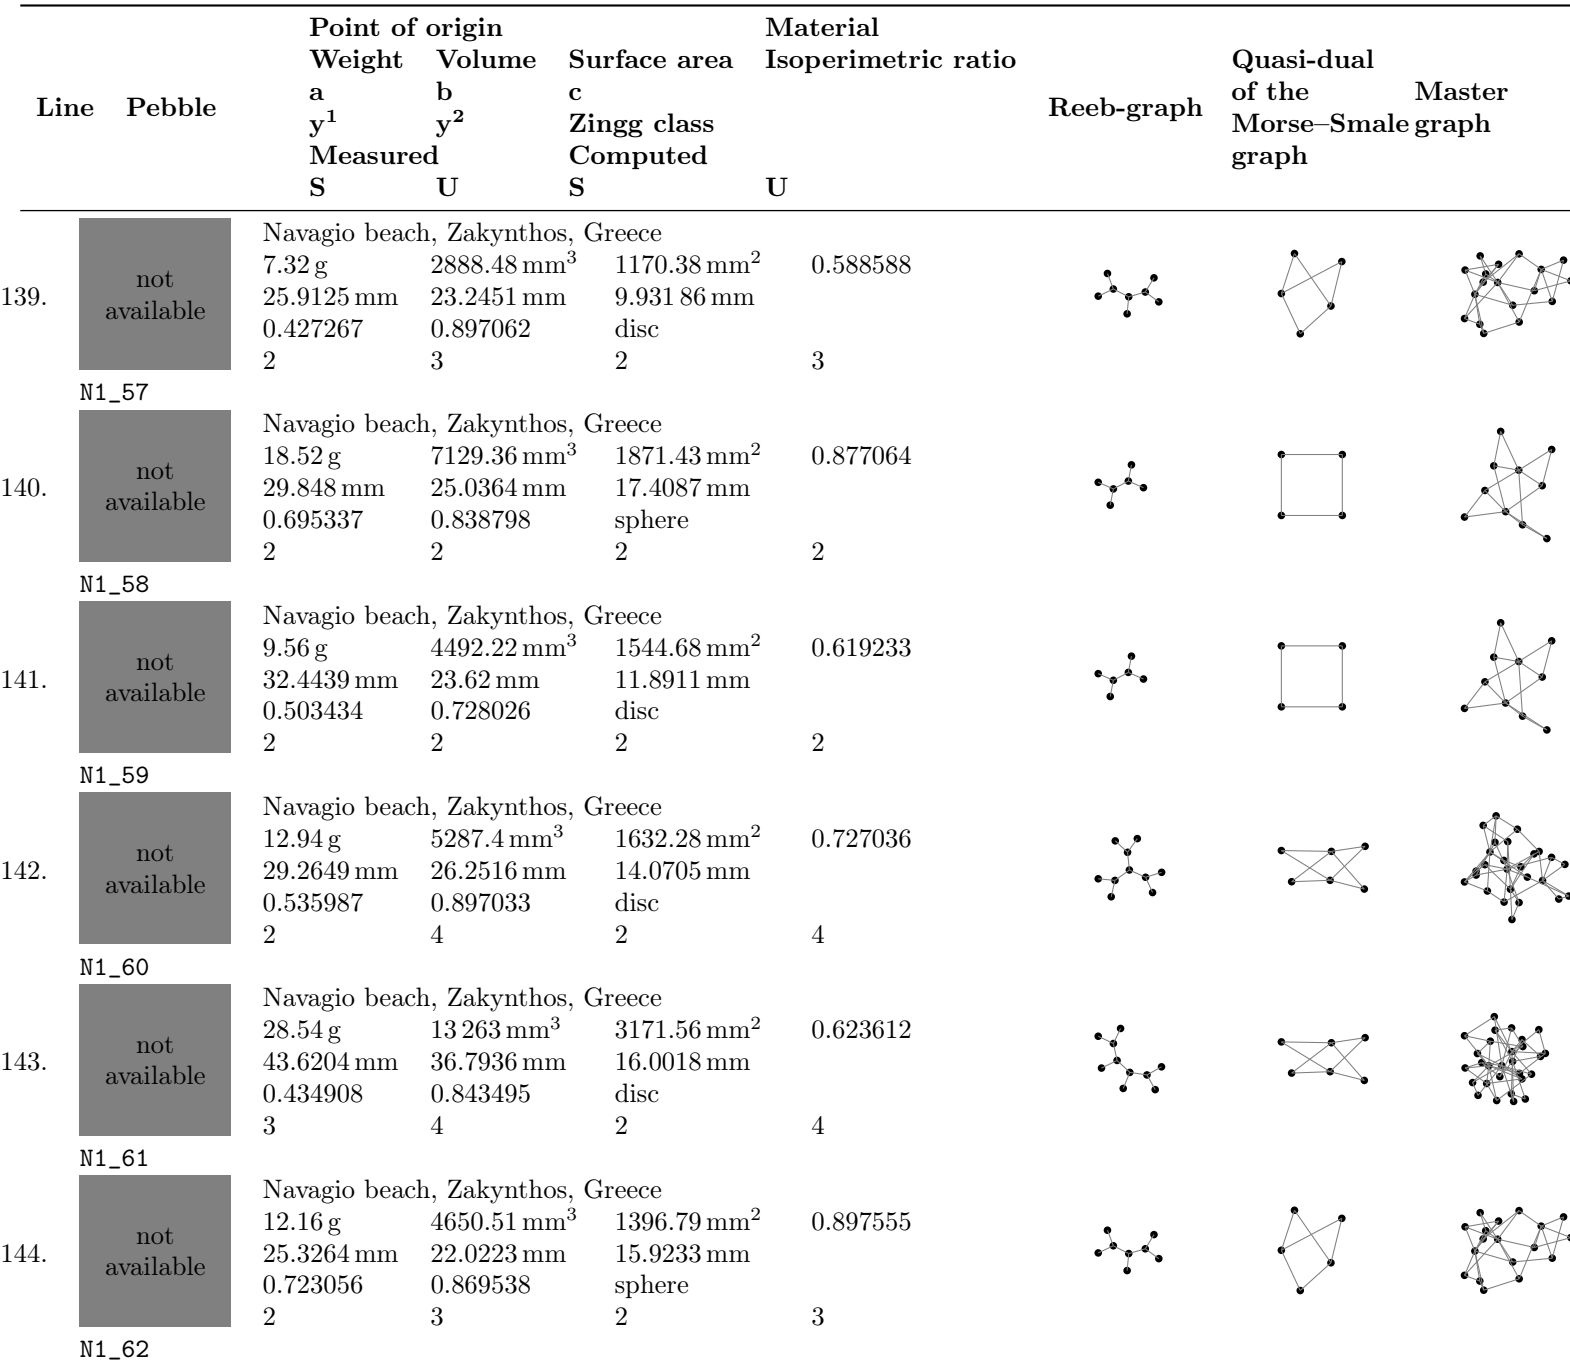   | 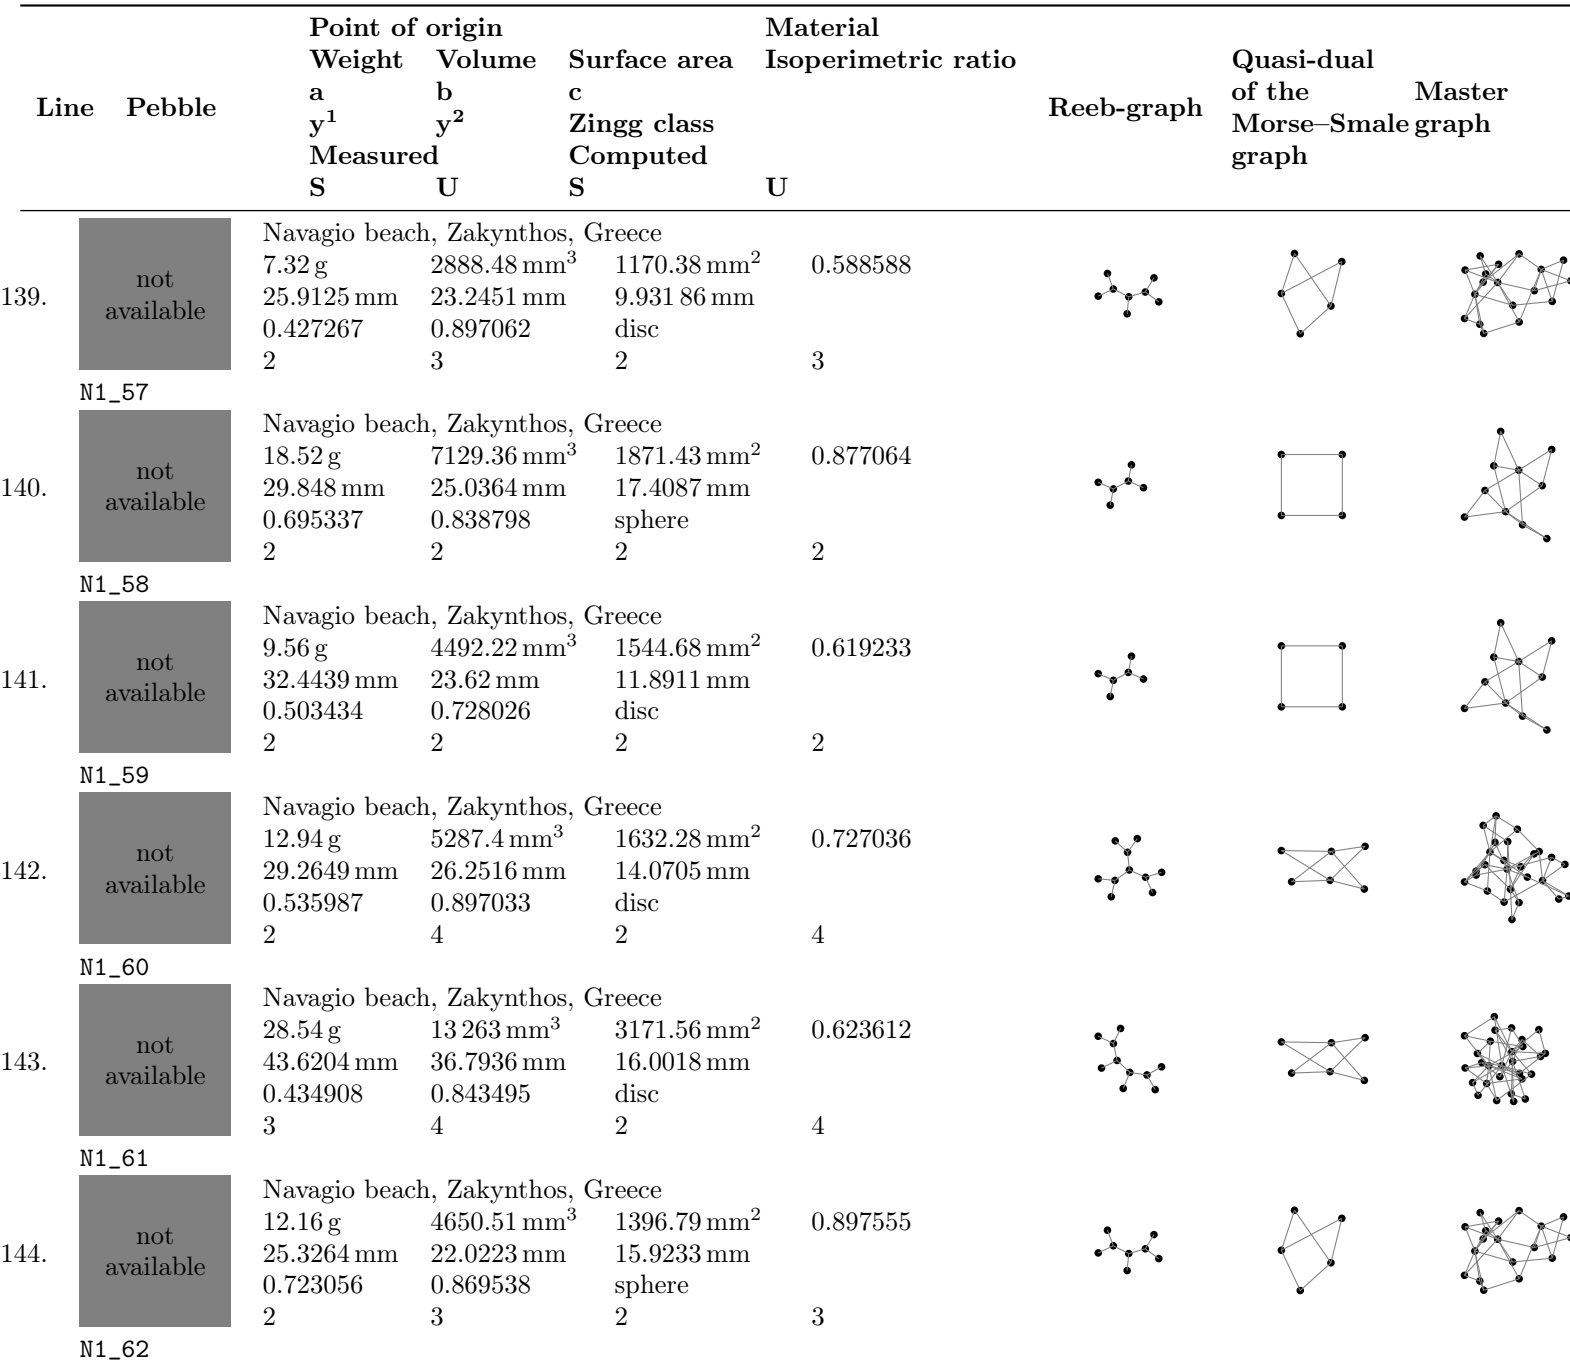   | 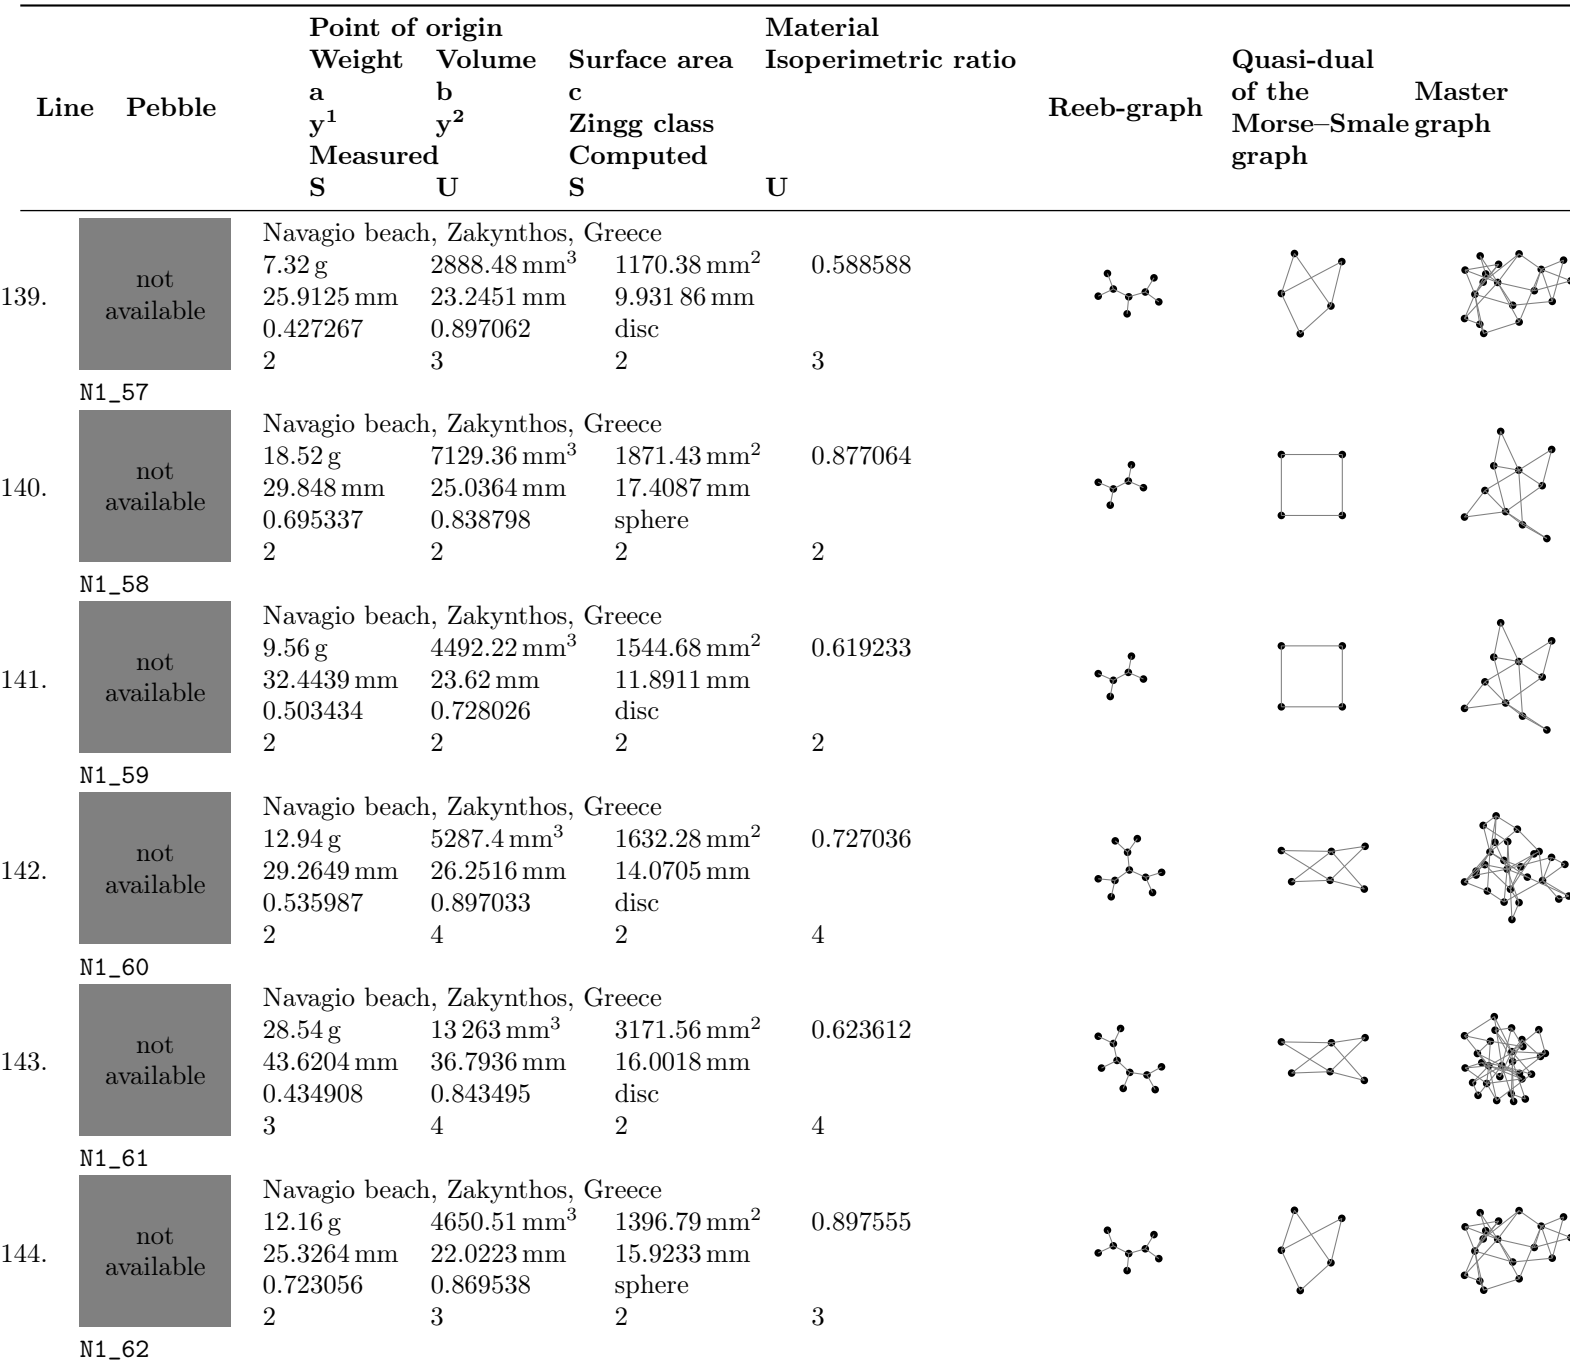   |
|      |                               | 7.32 g                           | 2888.48 mm <sup>3</sup> | 1170.38 mm <sup>2</sup>      |                                      |                                                                                       |                                                                                       |                                                                                       |
|      |                               | 25.9125 mm                       | 23.2451 mm              | 9.931 86 mm                  |                                      |                                                                                       |                                                                                       |                                                                                       |
|      |                               | 0.427267                         | 0.897062                | disc                         |                                      |                                                                                       |                                                                                       |                                                                                       |
|      |                               | 2                                | 3                       | 2                            |                                      |                                                                                       |                                                                                       |                                                                                       |
|      |                               |                                  |                         |                              |                                      |                                                                                       |                                                                                       |                                                                                       |
| 140. | not<br>available<br><br>N1_58 | Navagio beach, Zakynthos, Greece |                         |                              | 0.877064<br><br><br><br>2            | 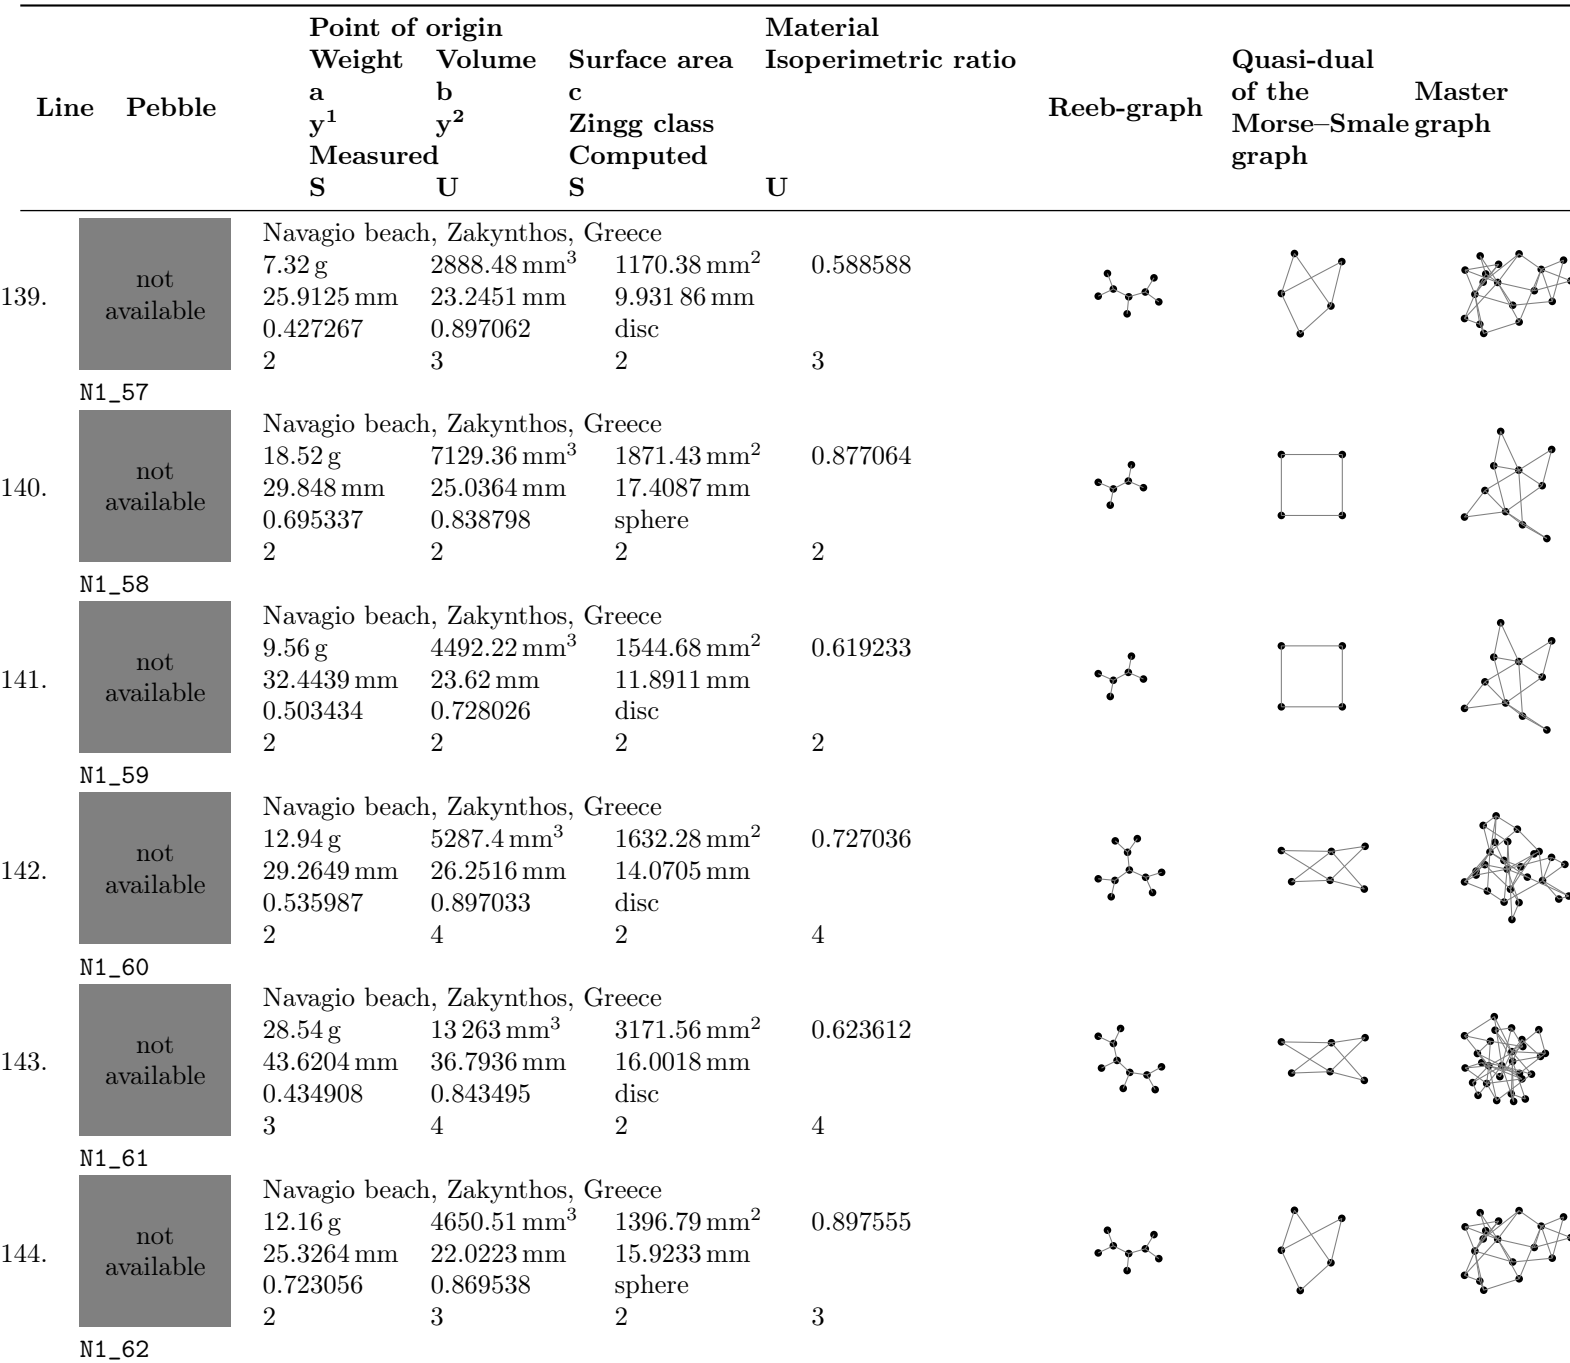   | 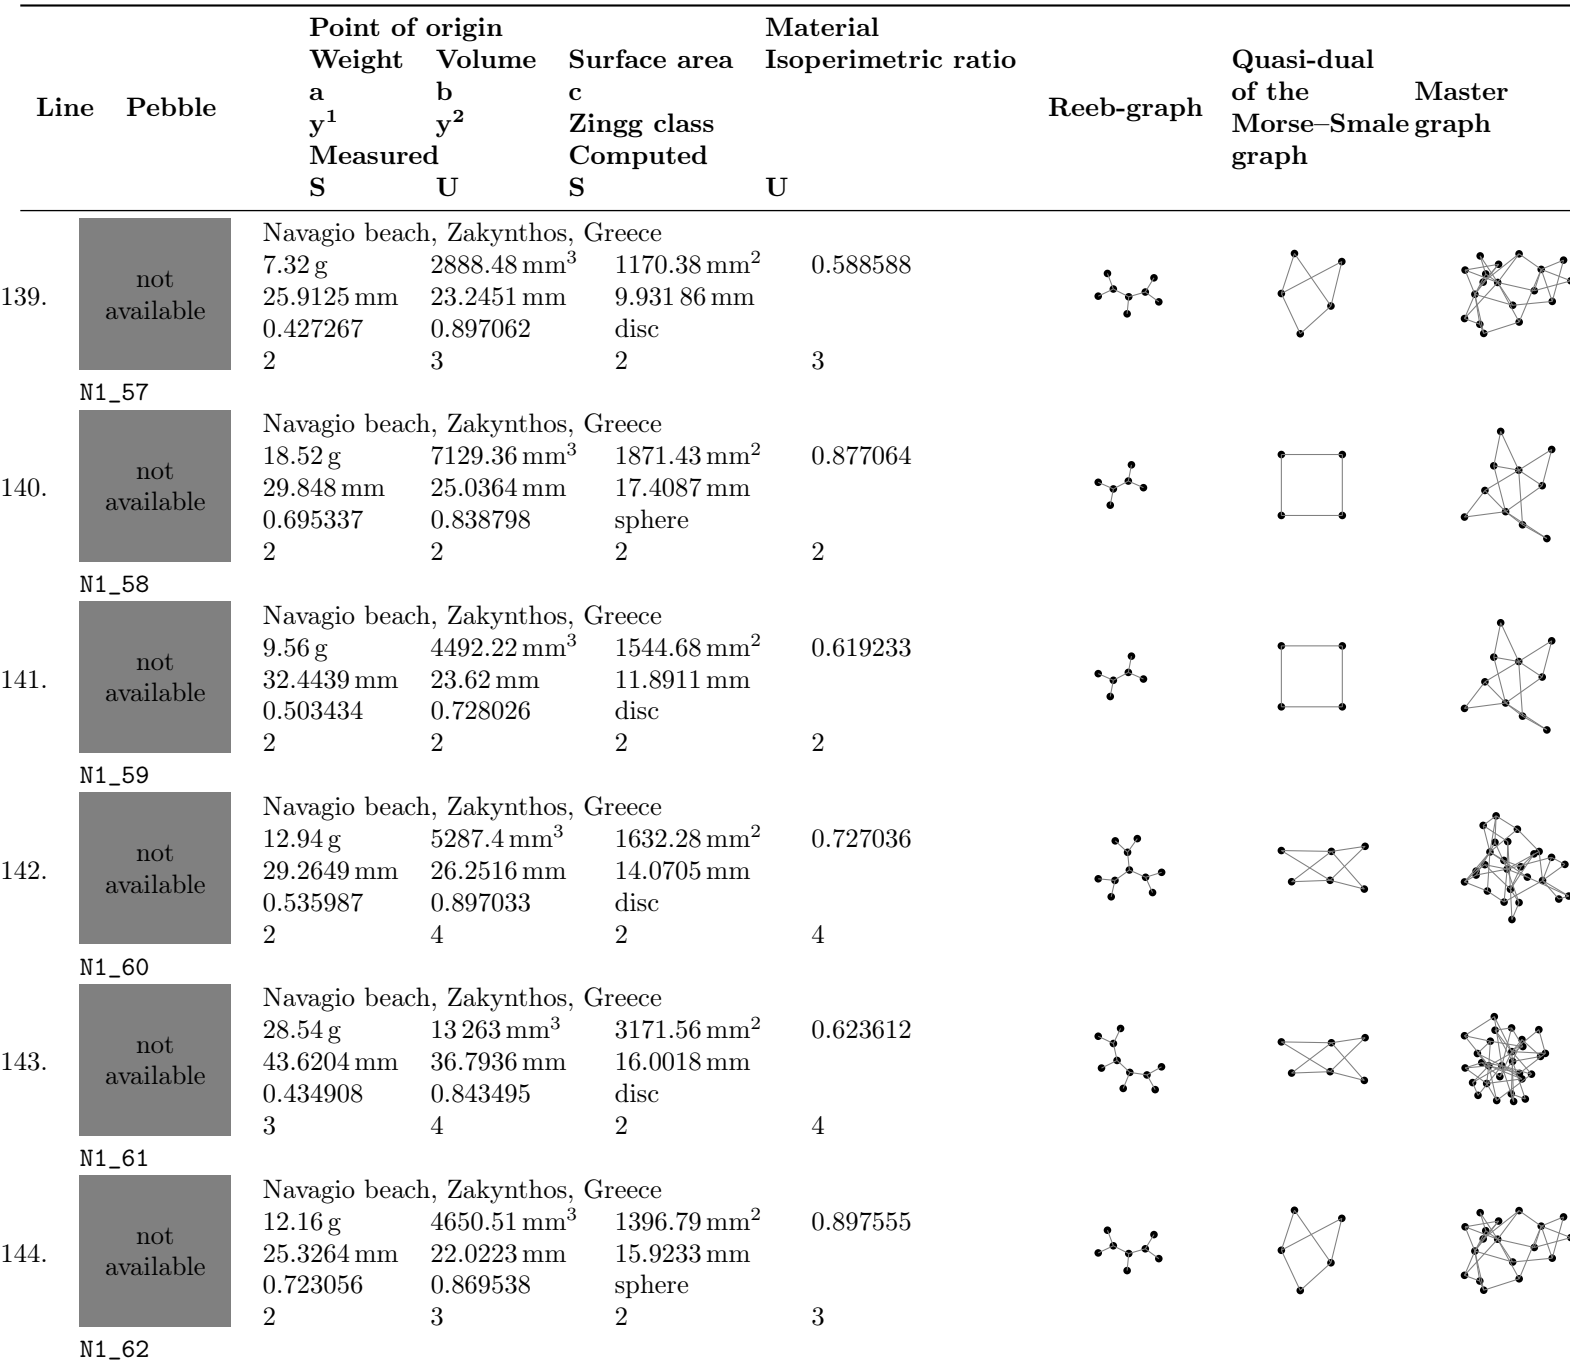   | 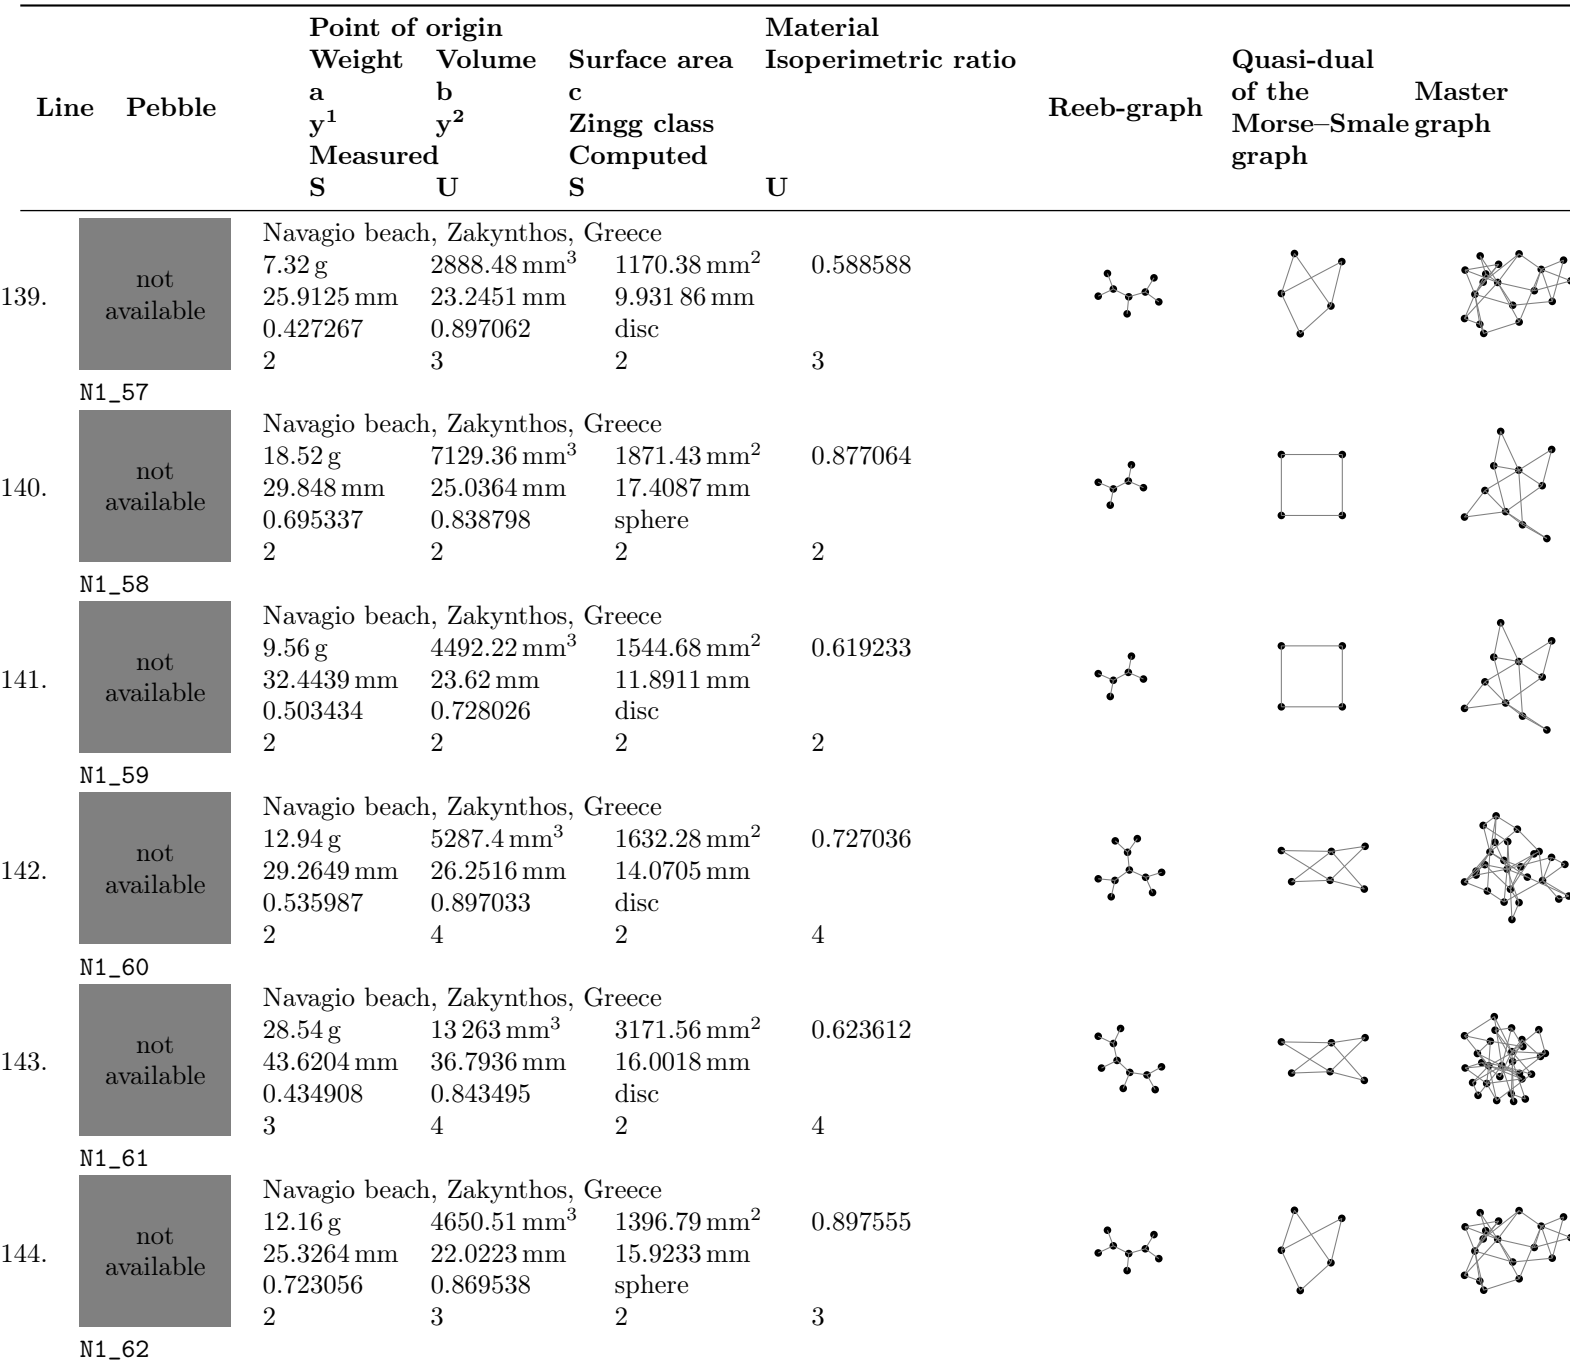   |
|      |                               | 18.52 g                          | 7129.36 mm <sup>3</sup> | 1871.43 mm <sup>2</sup>      |                                      |                                                                                       |                                                                                       |                                                                                       |
|      |                               | 29.848 mm                        | 25.0364 mm              | 17.4087 mm                   |                                      |                                                                                       |                                                                                       |                                                                                       |
|      |                               | 0.695337                         | 0.838798                | sphere                       |                                      |                                                                                       |                                                                                       |                                                                                       |
|      |                               | 2                                | 2                       | 2                            |                                      |                                                                                       |                                                                                       |                                                                                       |
|      |                               |                                  |                         |                              |                                      |                                                                                       |                                                                                       |                                                                                       |
| 141. | not<br>available<br><br>N1_59 | Navagio beach, Zakynthos, Greece |                         |                              | 0.619233<br><br><br><br>2            | 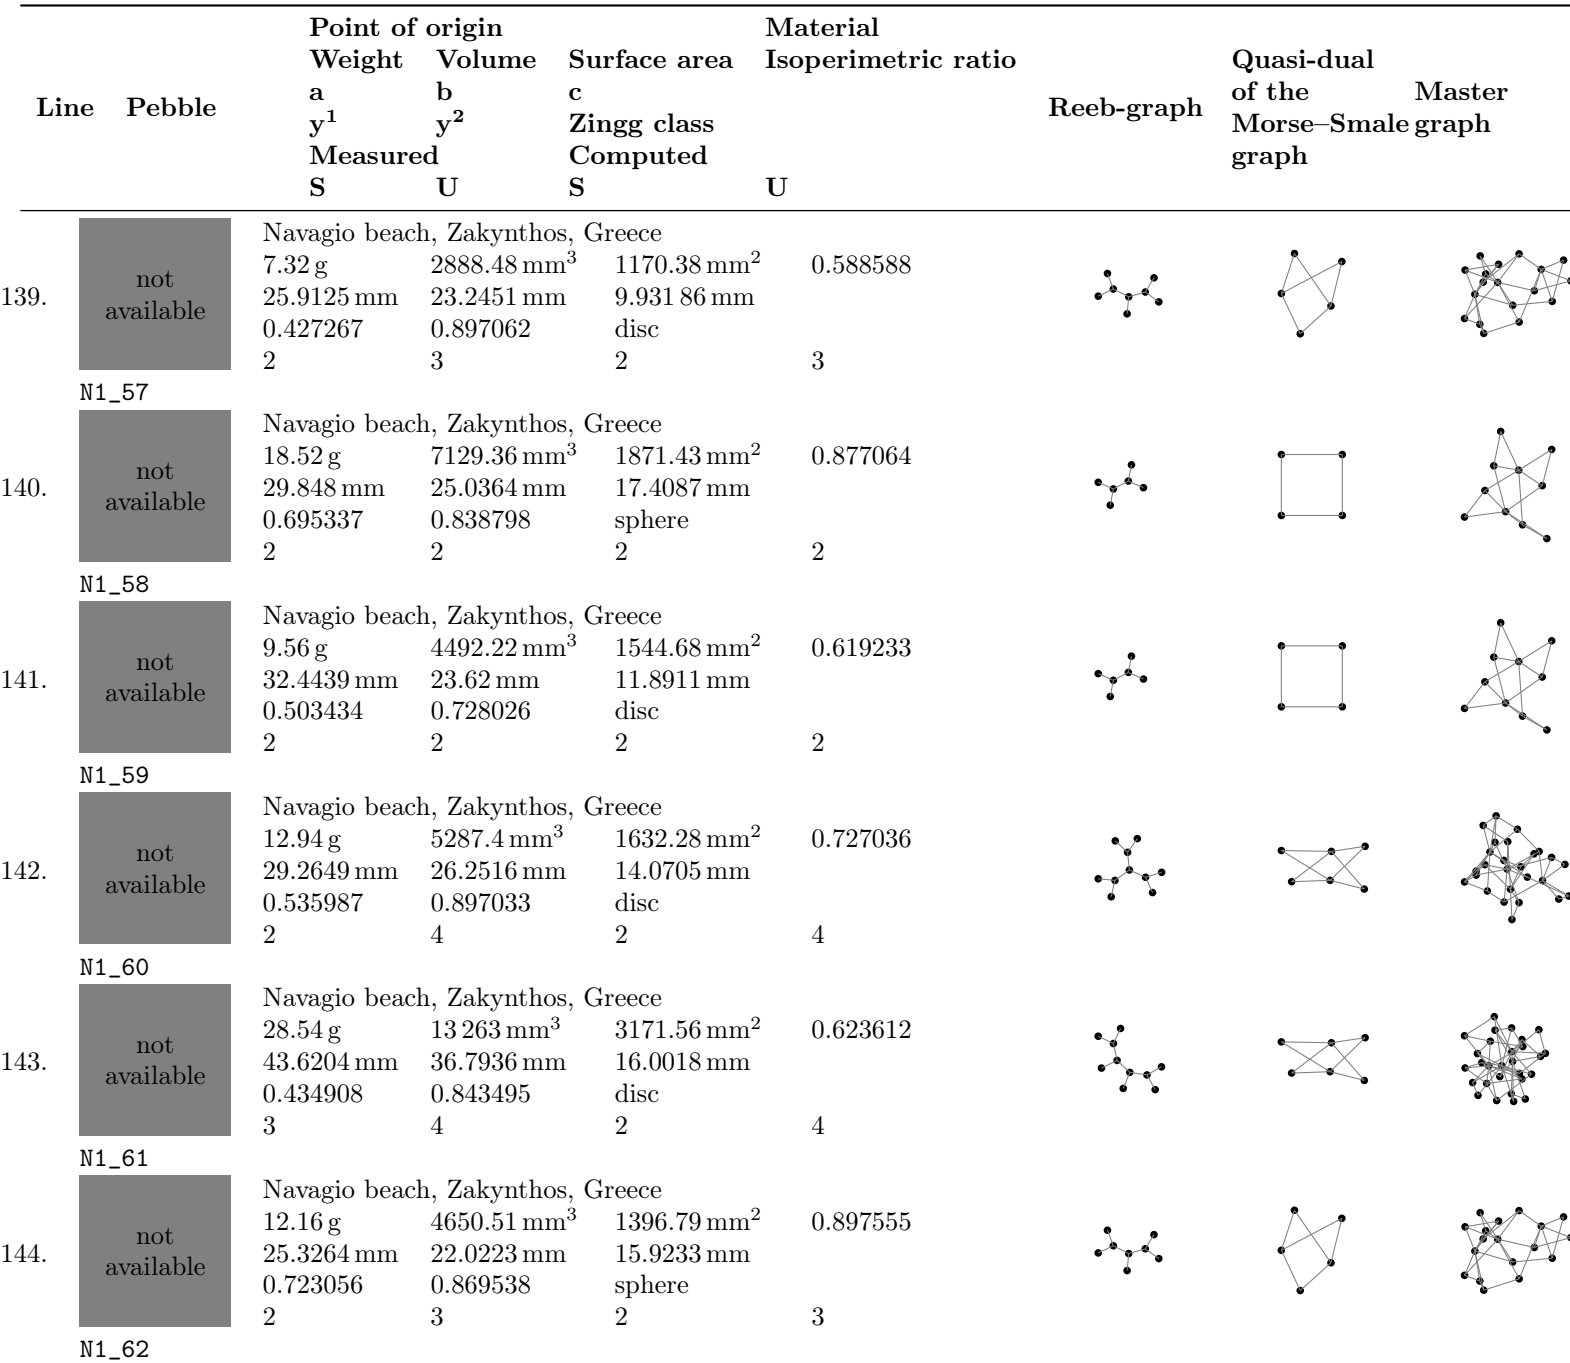   | 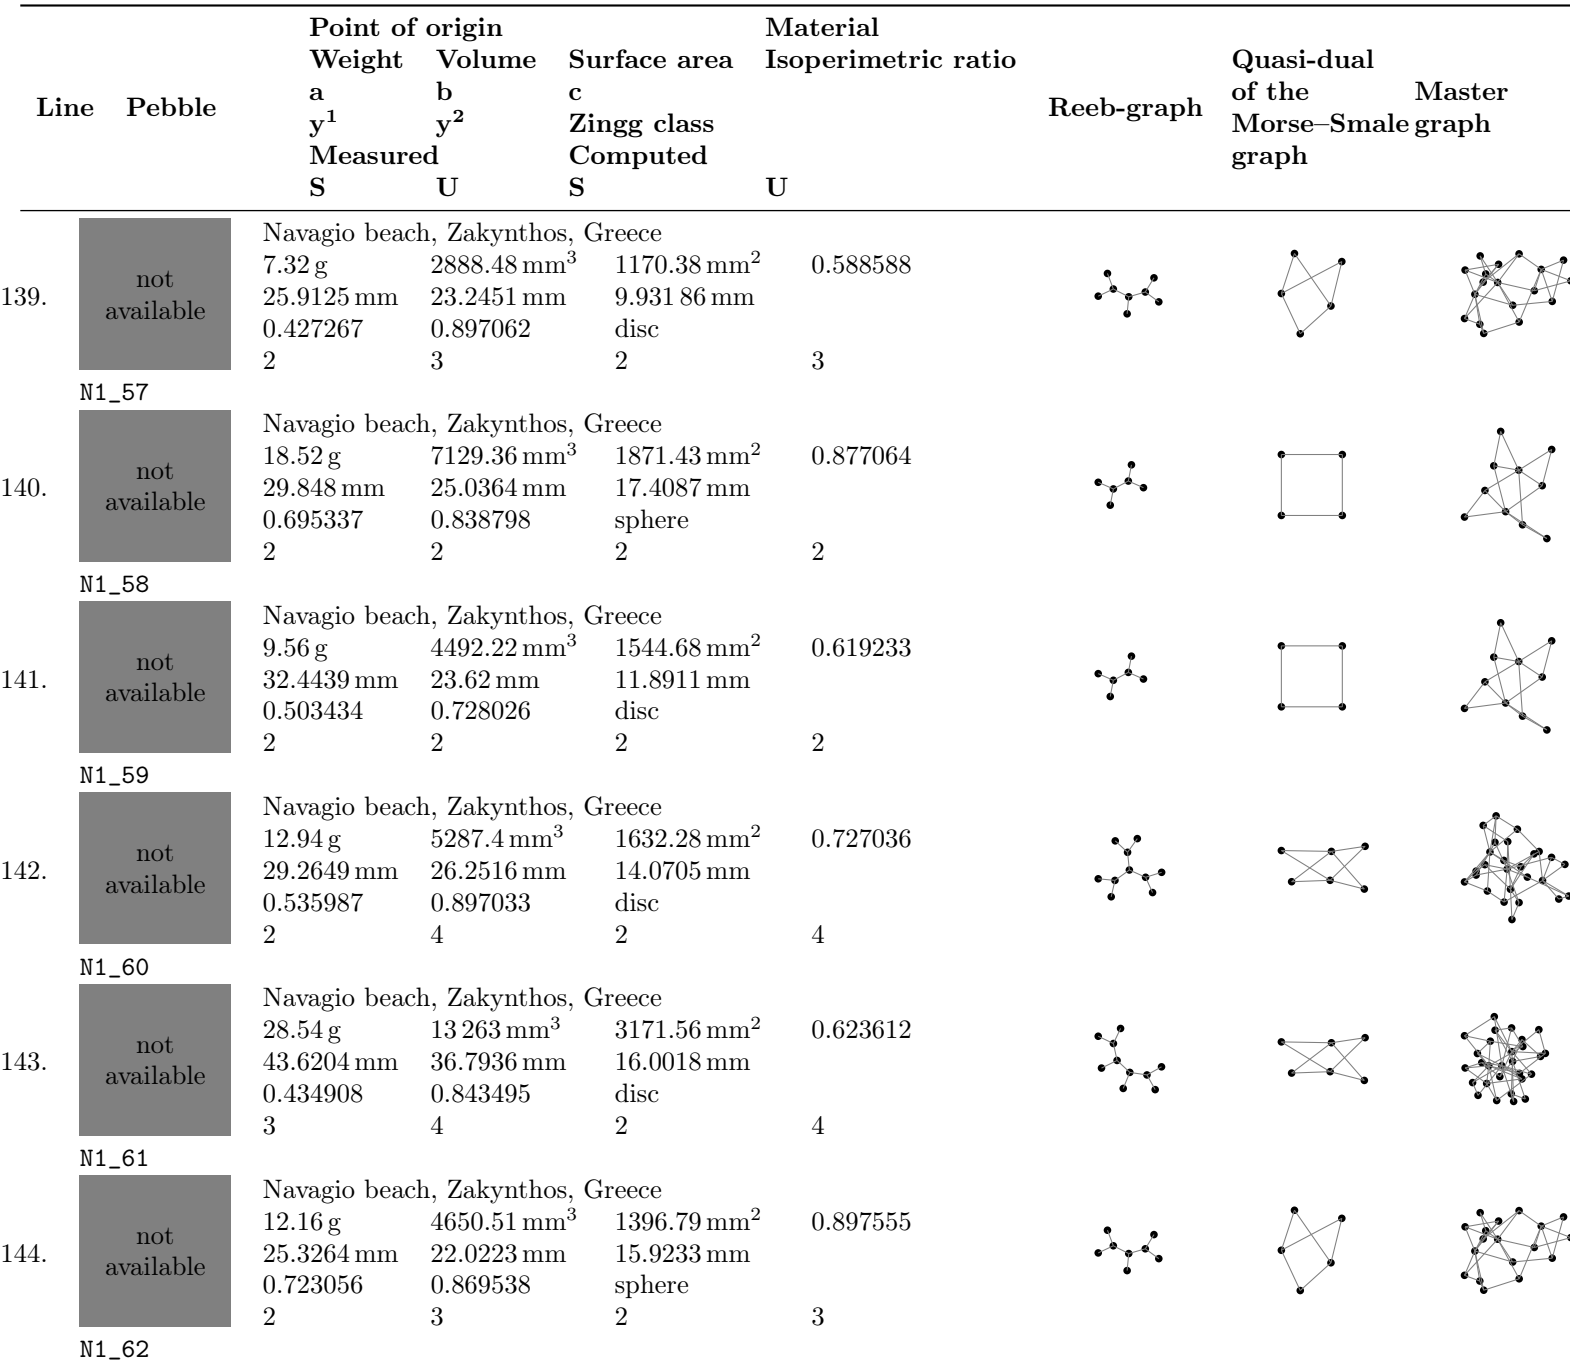   | 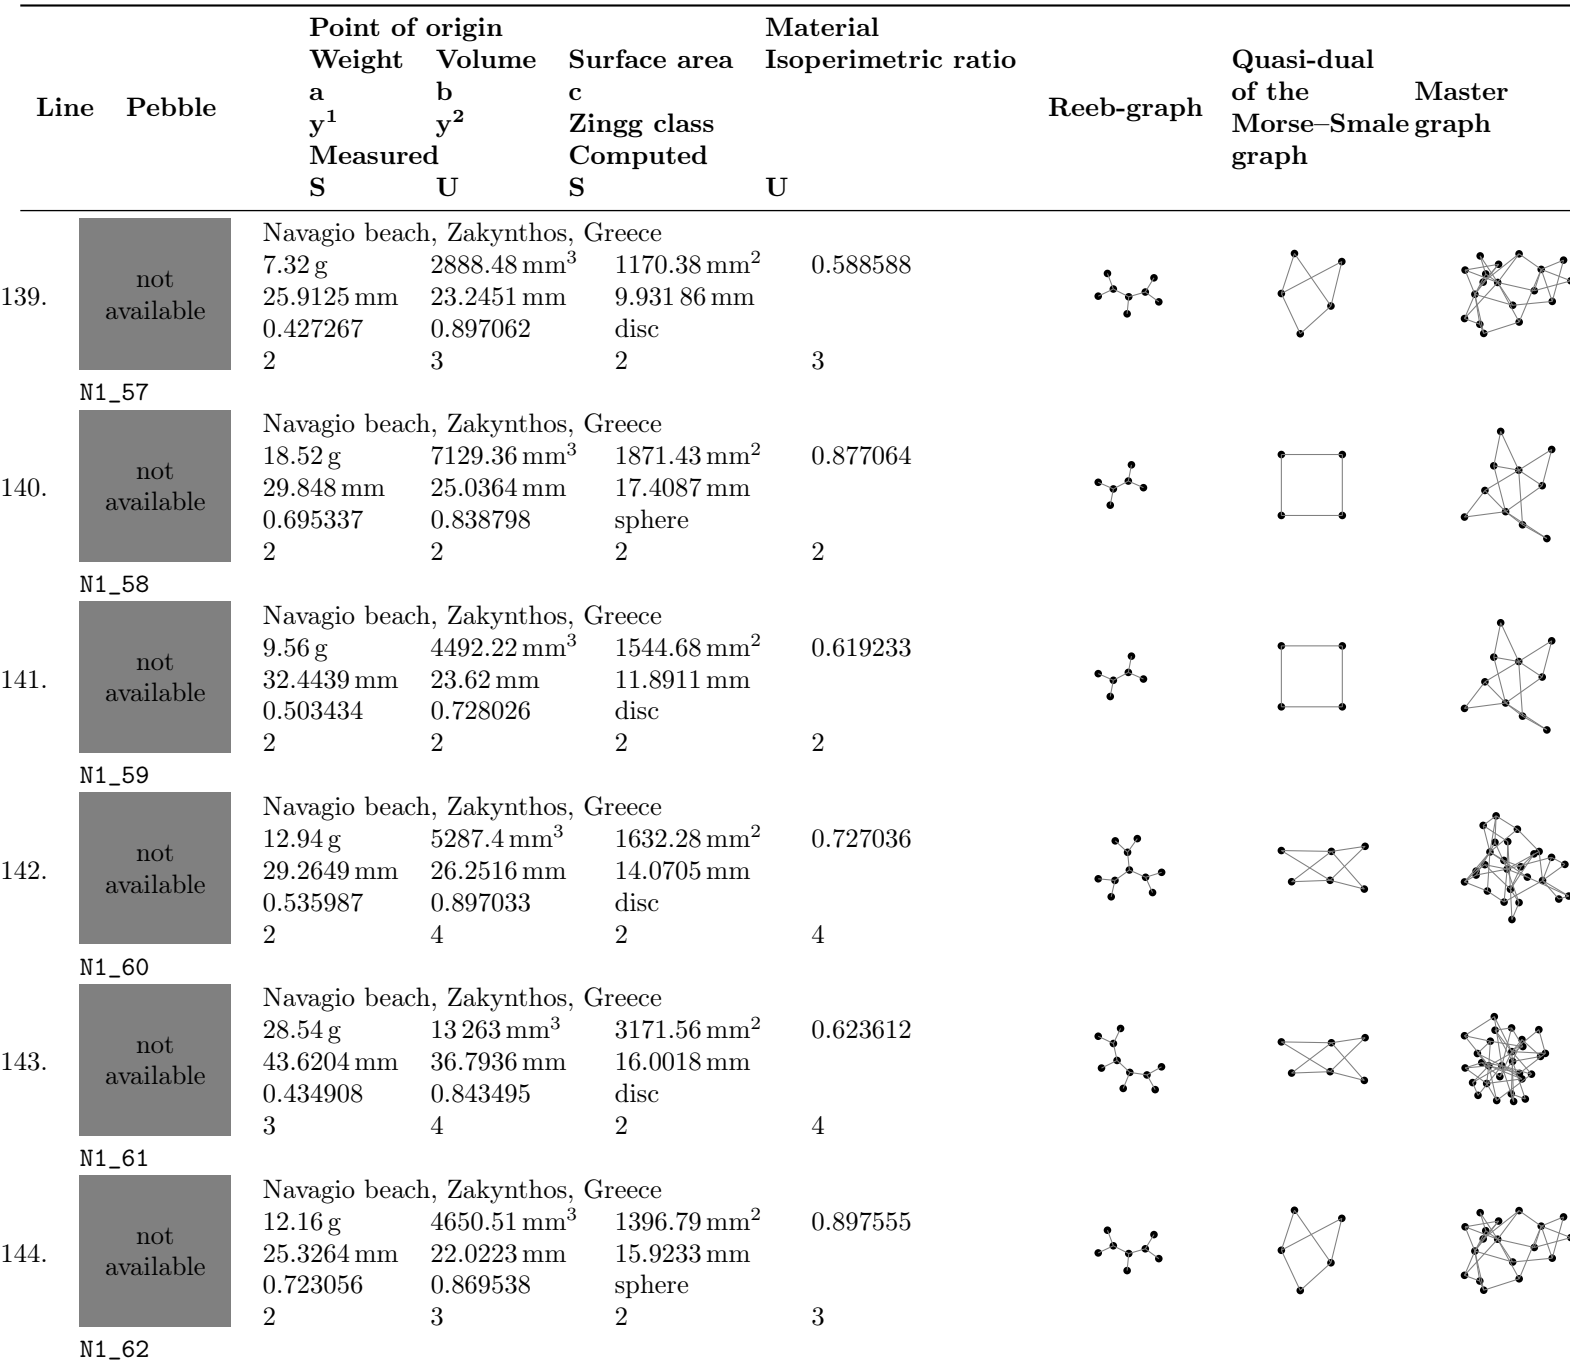   |
|      |                               | 9.56 g                           | 4492.22 mm <sup>3</sup> | 1544.68 mm <sup>2</sup>      |                                      |                                                                                       |                                                                                       |                                                                                       |
|      |                               | 32.4439 mm                       | 23.62 mm                | 11.8911 mm                   |                                      |                                                                                       |                                                                                       |                                                                                       |
|      |                               | 0.503434                         | 0.728026                | disc                         |                                      |                                                                                       |                                                                                       |                                                                                       |
|      |                               | 2                                | 2                       | 2                            |                                      |                                                                                       |                                                                                       |                                                                                       |
|      |                               |                                  |                         |                              |                                      |                                                                                       |                                                                                       |                                                                                       |
| 142. | not<br>available<br><br>N1_60 | Navagio beach, Zakynthos, Greece |                         |                              | 0.727036<br><br><br><br>4            | 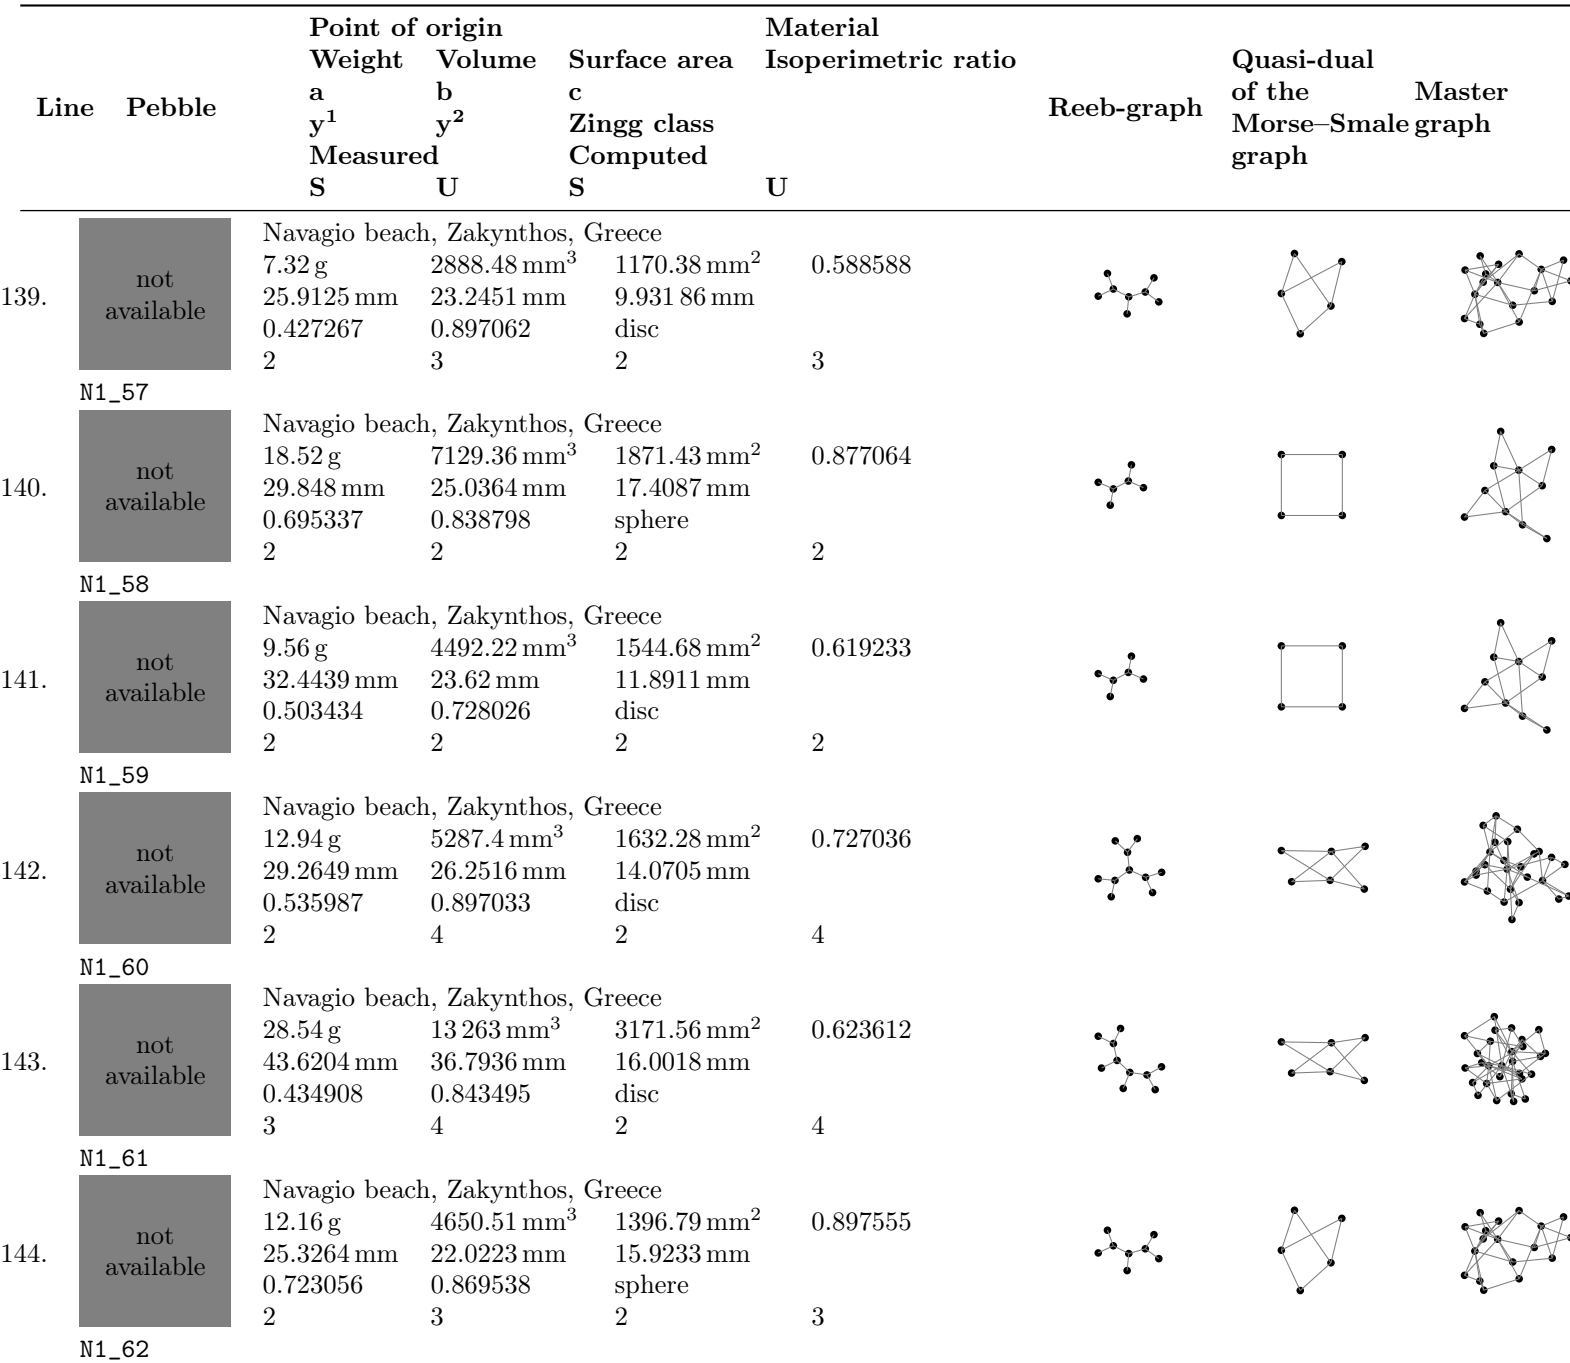  | 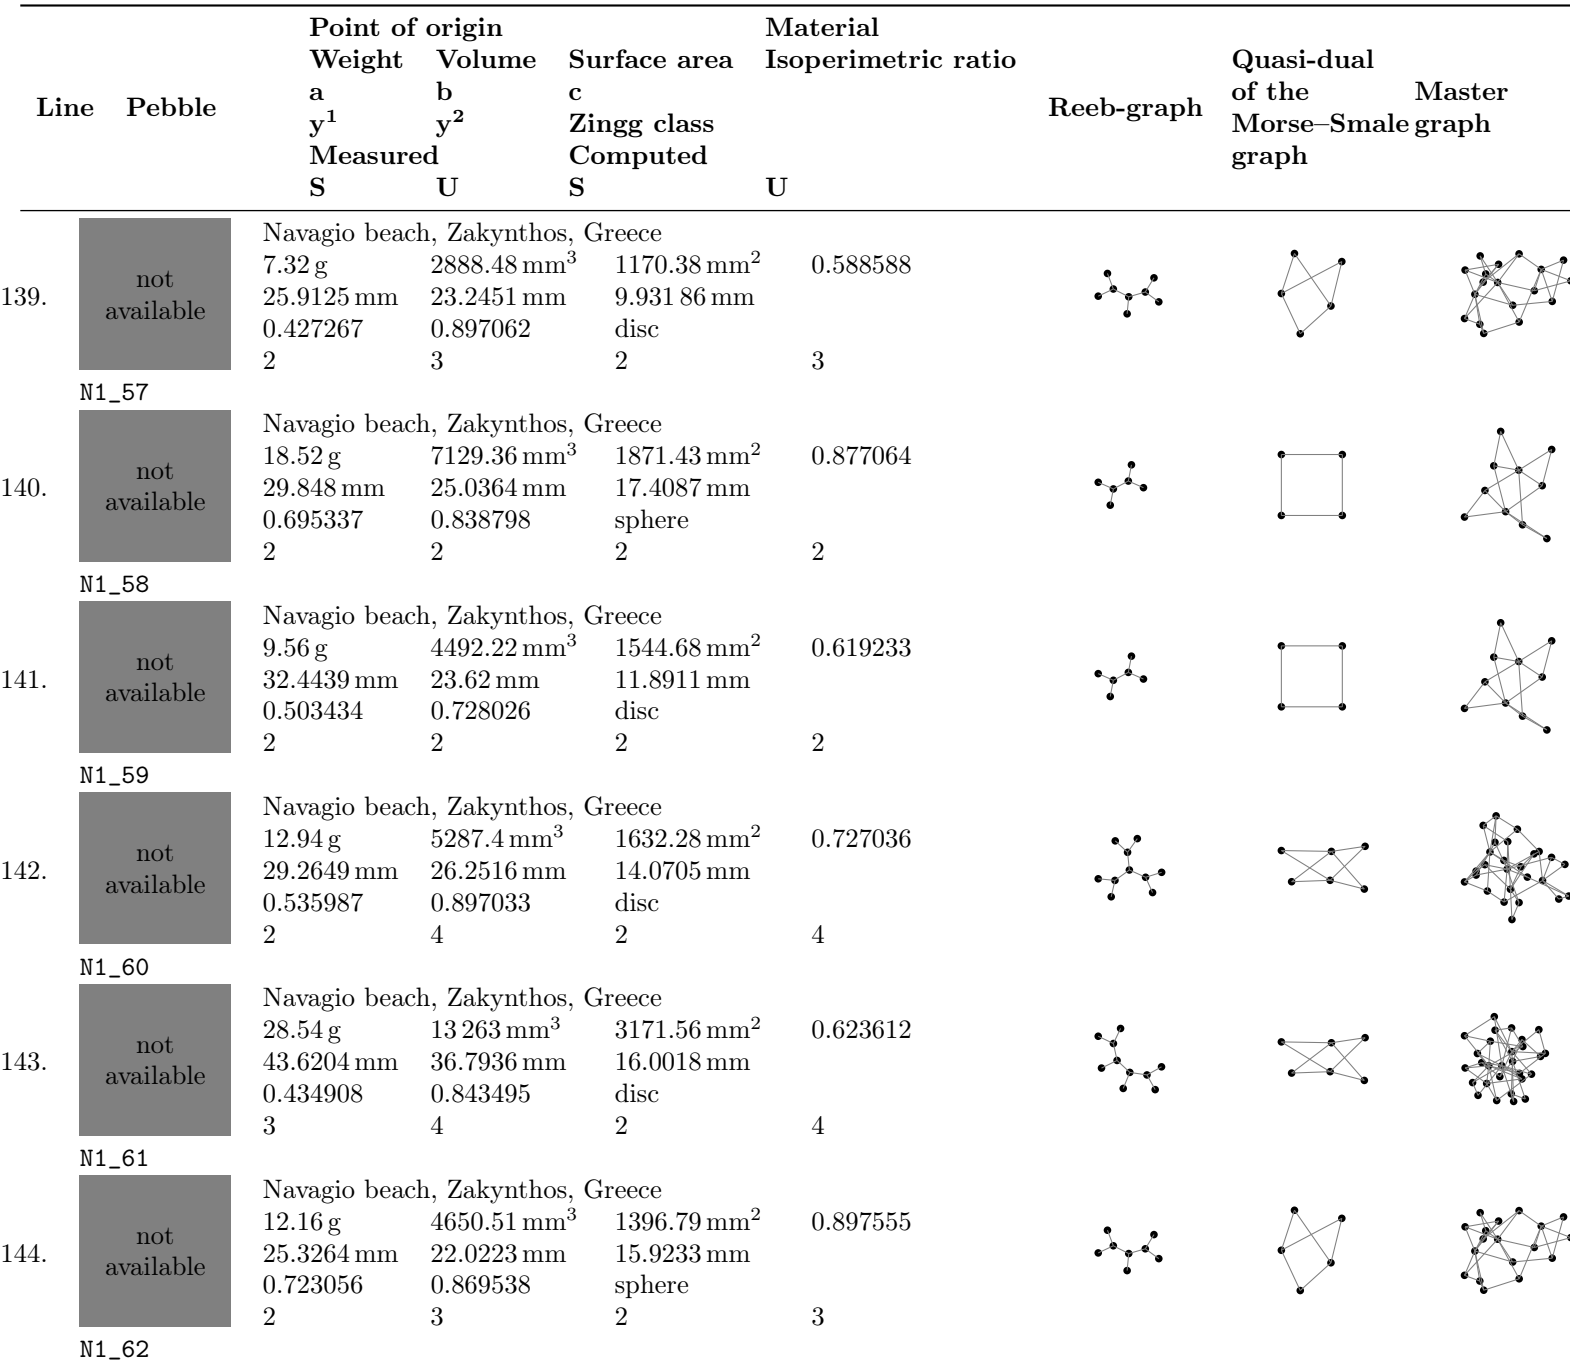  | 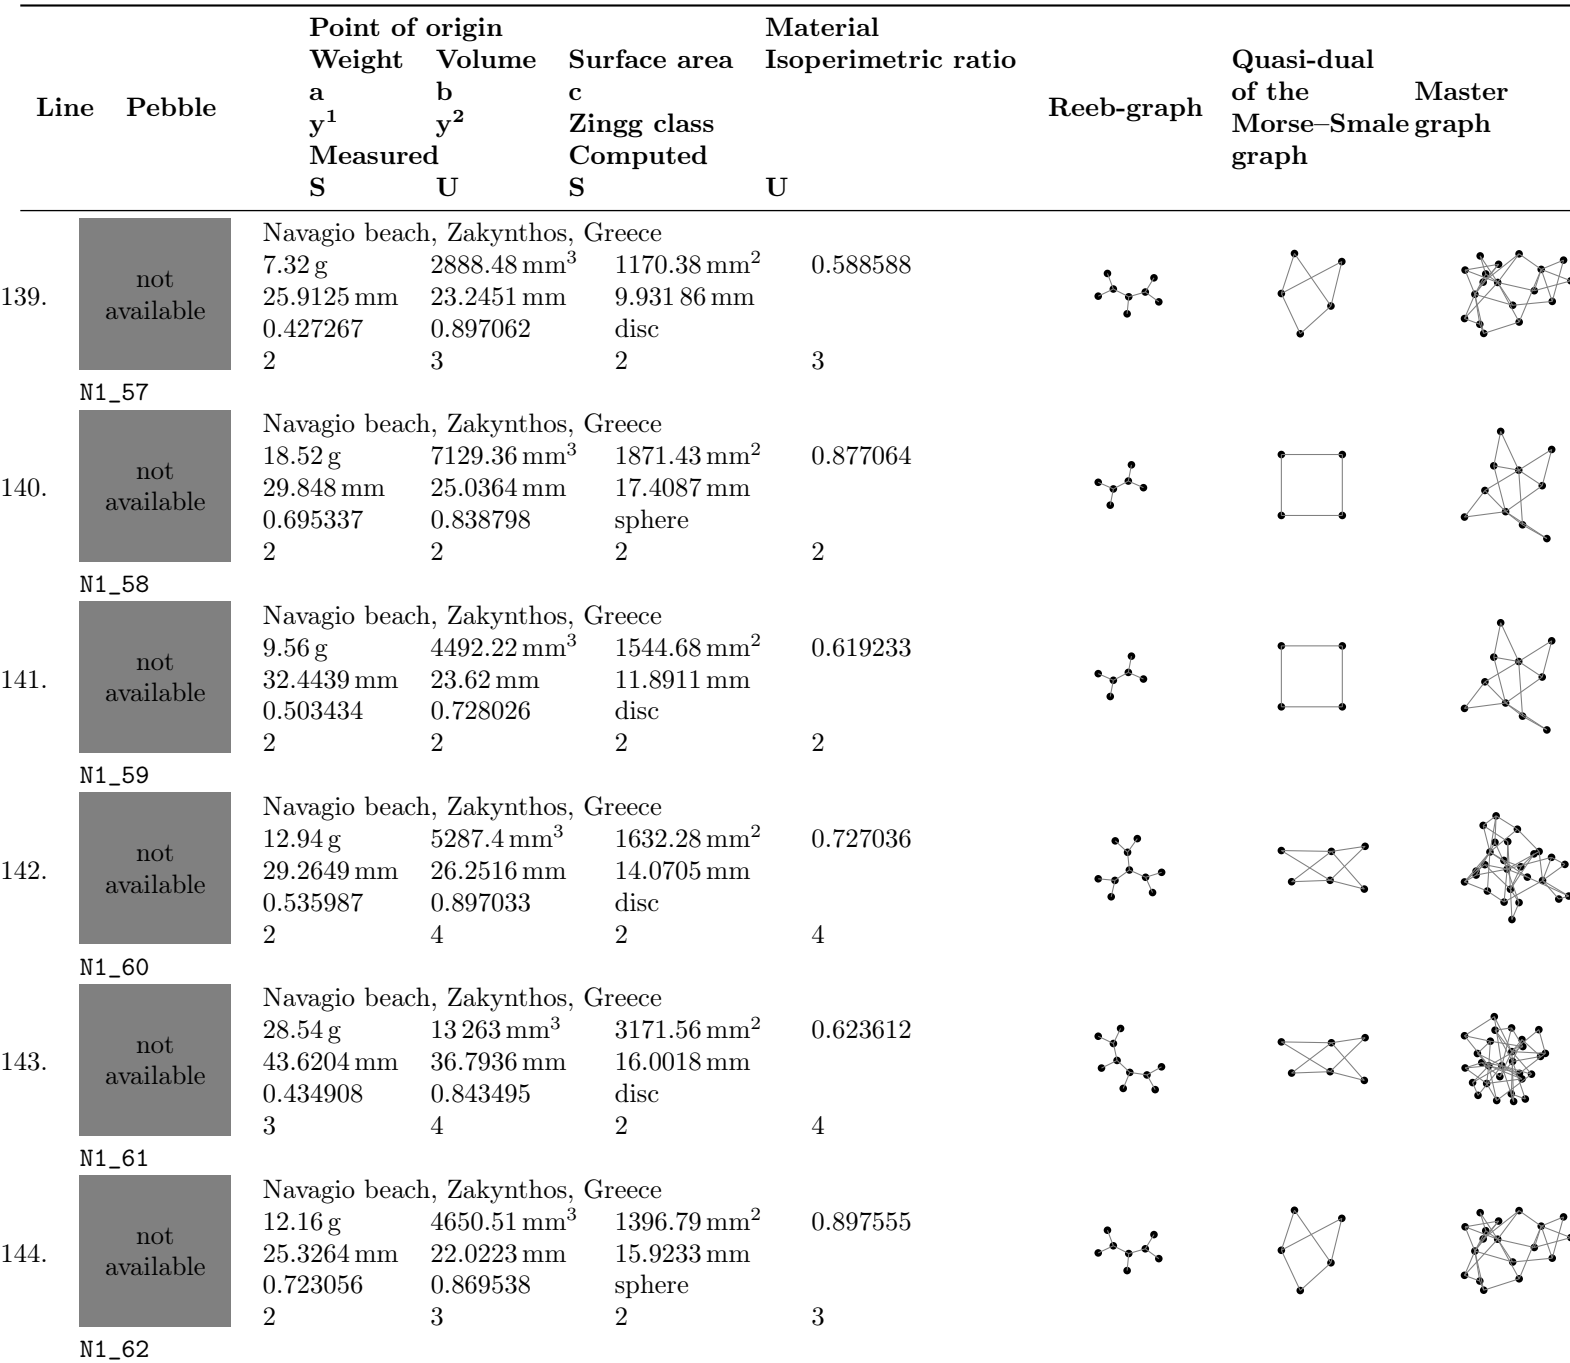  |
|      |                               | 12.94 g                          | 5287.4 mm <sup>3</sup>  | 1632.28 mm <sup>2</sup>      |                                      |                                                                                       |                                                                                       |                                                                                       |
|      |                               | 29.2649 mm                       | 26.2516 mm              | 14.0705 mm                   |                                      |                                                                                       |                                                                                       |                                                                                       |
|      |                               | 0.535987                         | 0.897033                | disc                         |                                      |                                                                                       |                                                                                       |                                                                                       |
|      |                               | 2                                | 4                       | 2                            |                                      |                                                                                       |                                                                                       |                                                                                       |
|      |                               |                                  |                         |                              |                                      |                                                                                       |                                                                                       |                                                                                       |
| 143. | not<br>available<br><br>N1_61 | Navagio beach, Zakynthos, Greece |                         |                              | 0.623612<br><br><br><br>4            | 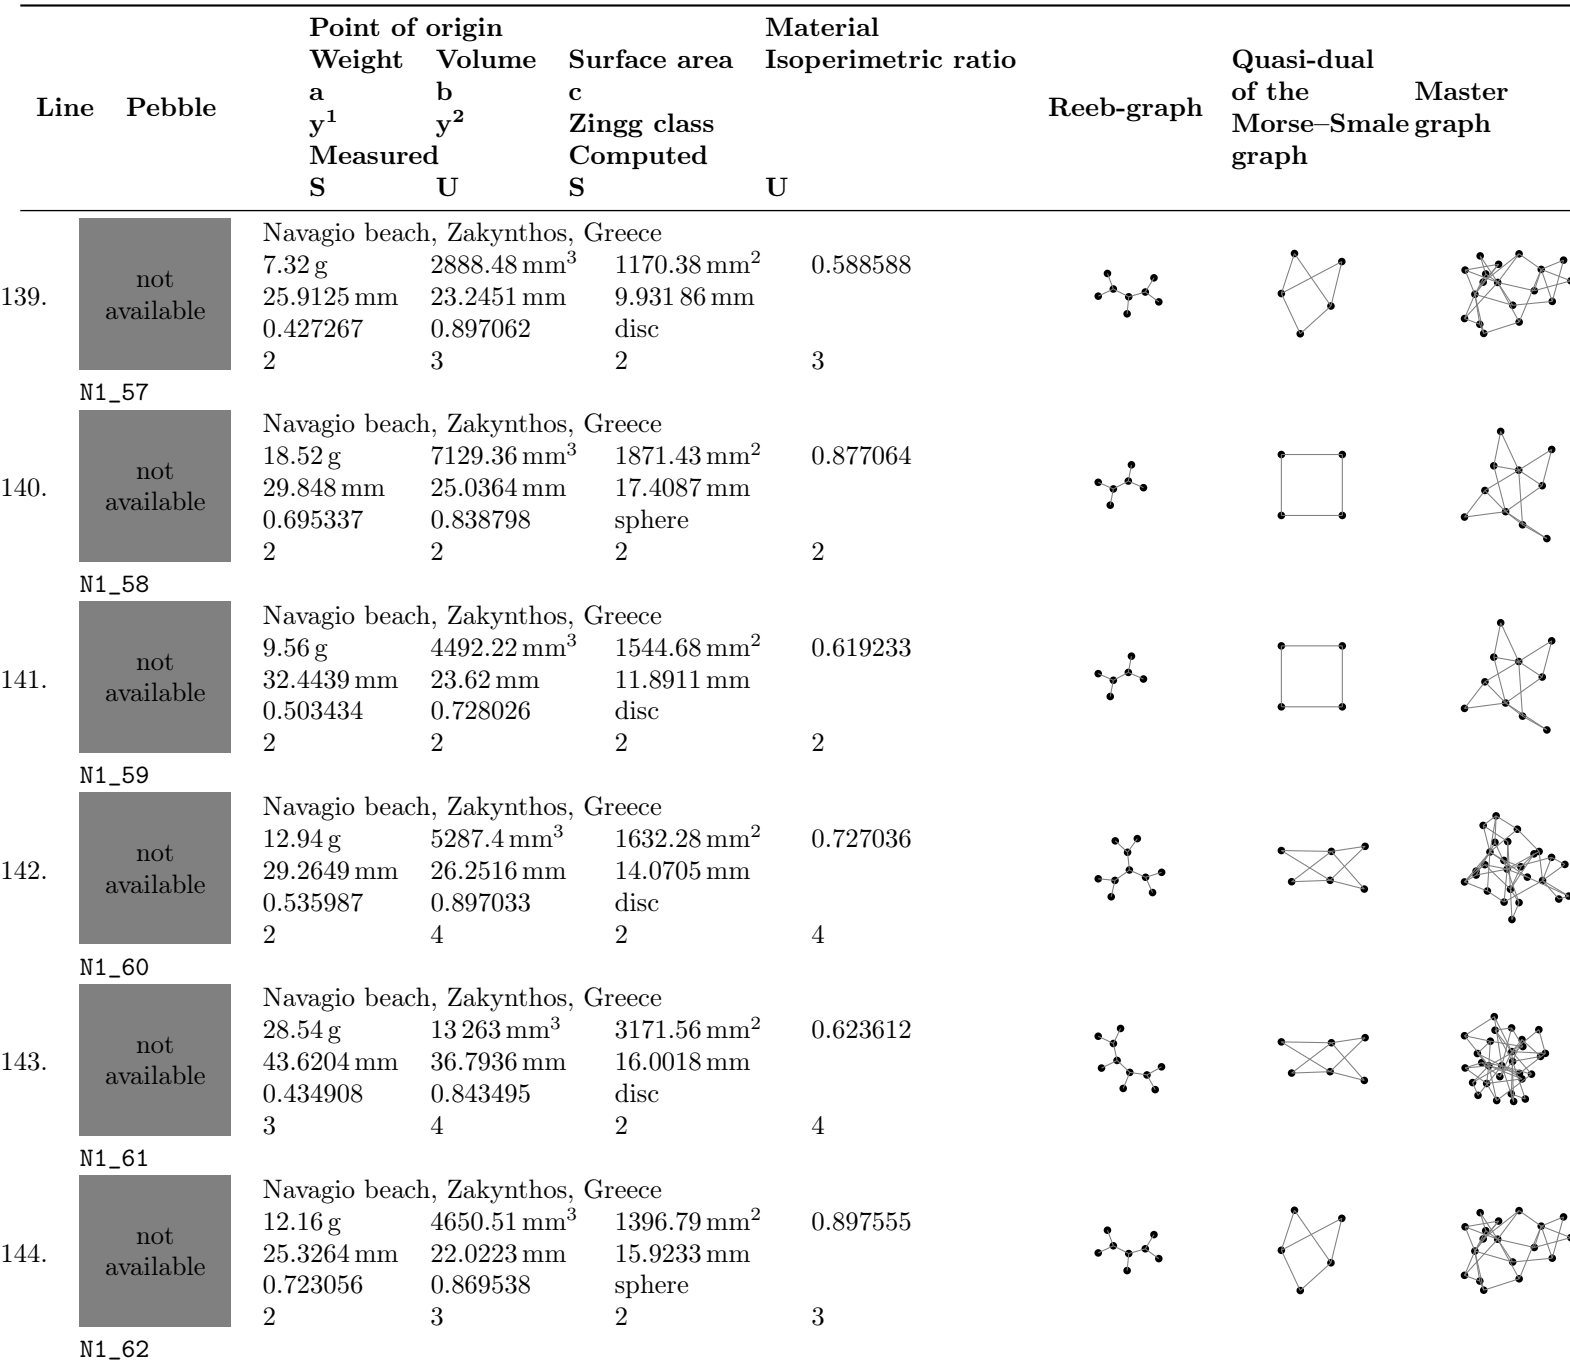 | 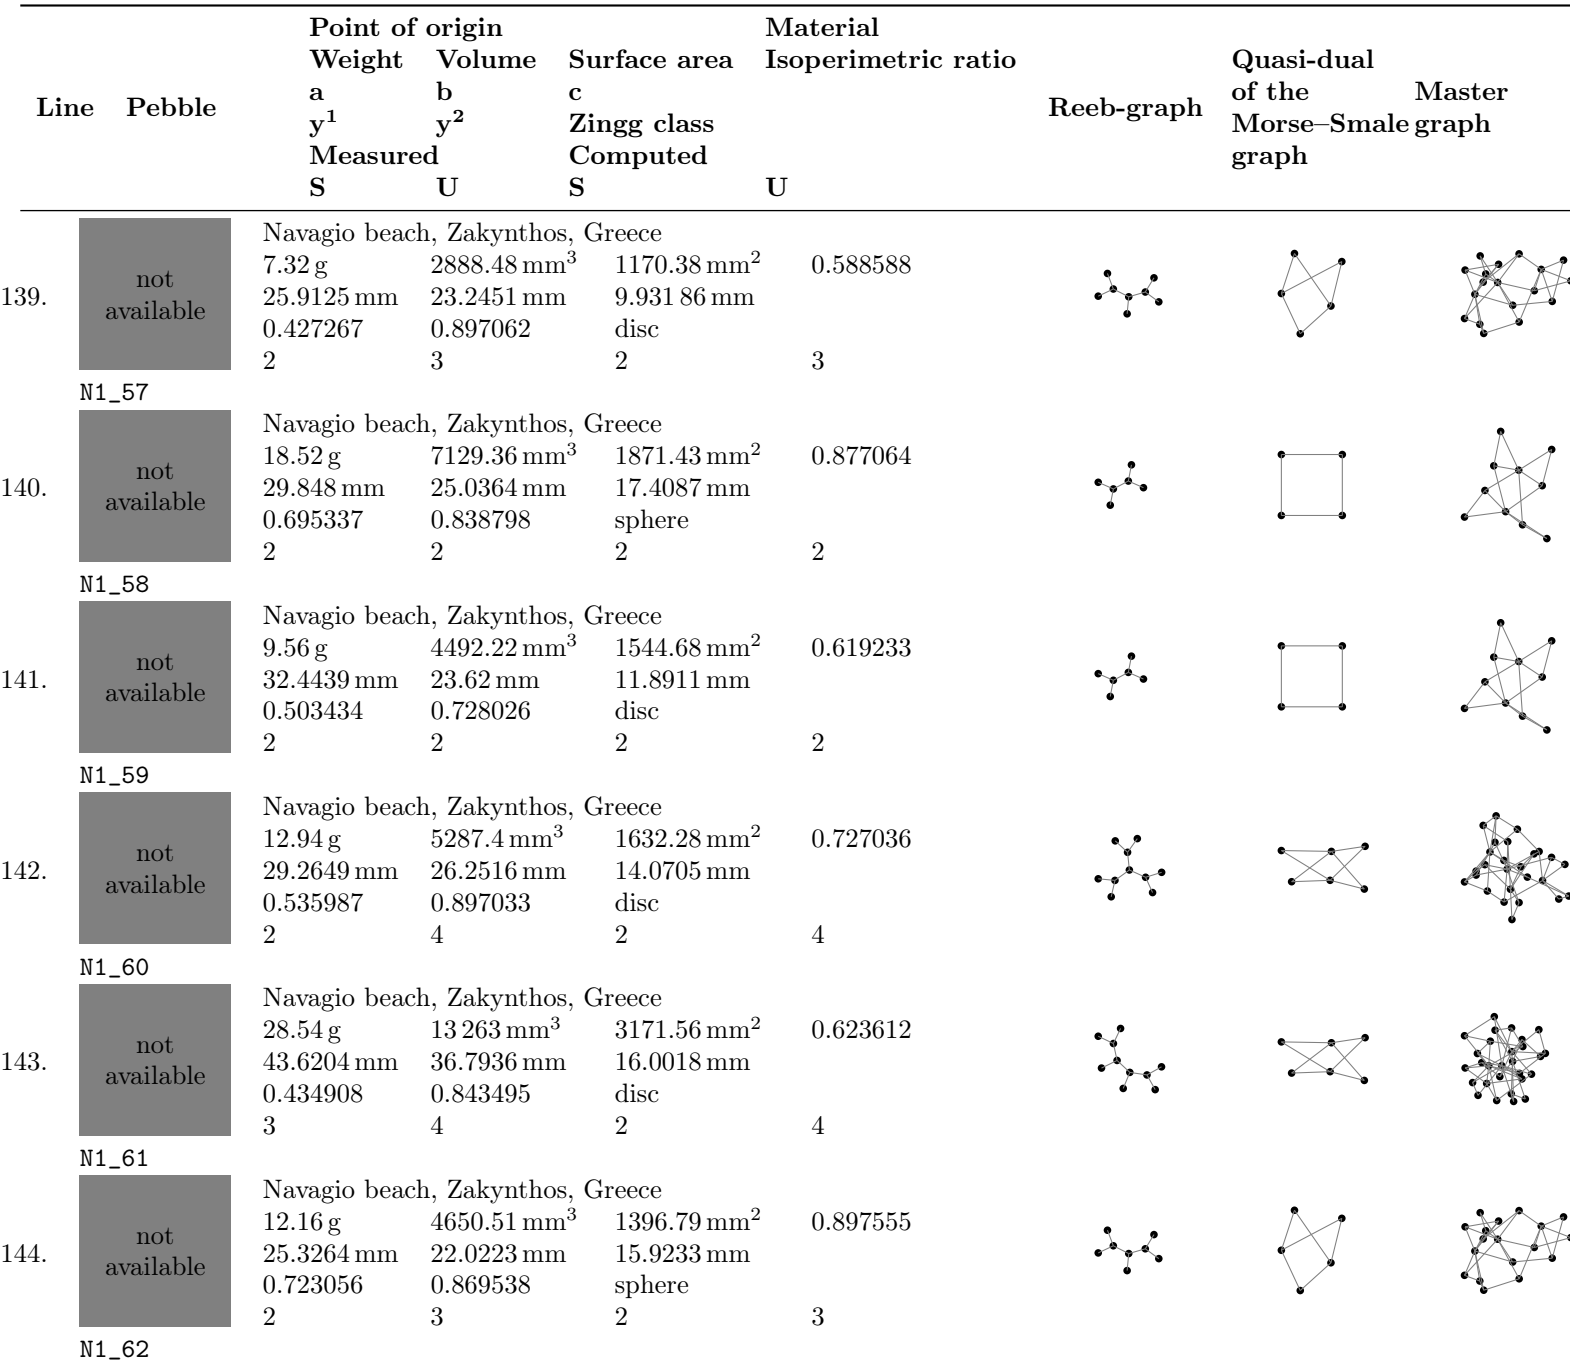 | 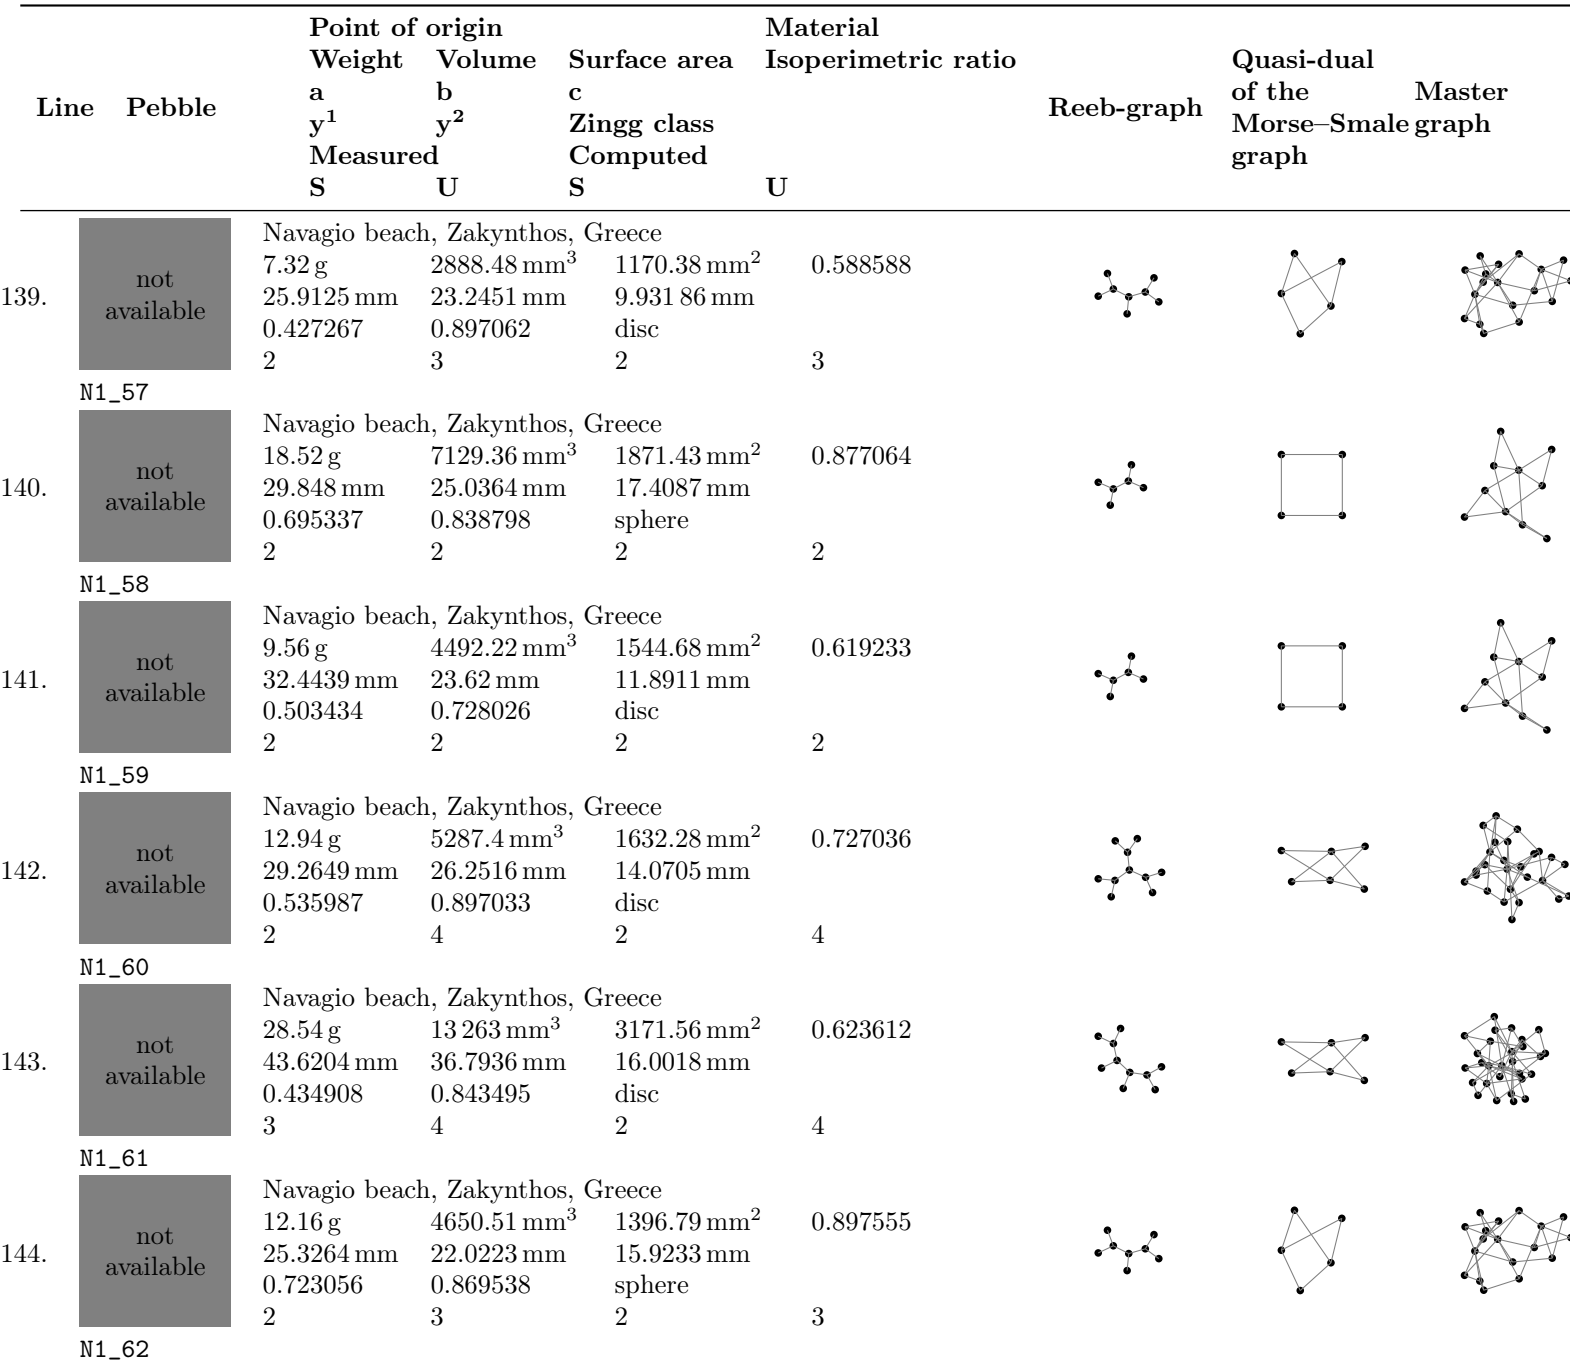 |
|      |                               | 28.54 g                          | 13 263 mm <sup>3</sup>  | 3171.56 mm <sup>2</sup>      |                                      |                                                                                       |                                                                                       |                                                                                       |
|      |                               | 43.6204 mm                       | 36.7936 mm              | 16.0018 mm                   |                                      |                                                                                       |                                                                                       |                                                                                       |
|      |                               | 0.434908                         | 0.843495                | disc                         |                                      |                                                                                       |                                                                                       |                                                                                       |
|      |                               | 3                                | 4                       | 2                            |                                      |                                                                                       |                                                                                       |                                                                                       |
|      |                               |                                  |                         |                              |                                      |                                                                                       |                                                                                       |                                                                                       |
| 144. | not<br>available<br><br>N1_62 | Navagio beach, Zakynthos, Greece |                         |                              | 0.897555<br><br><br><br>3            | 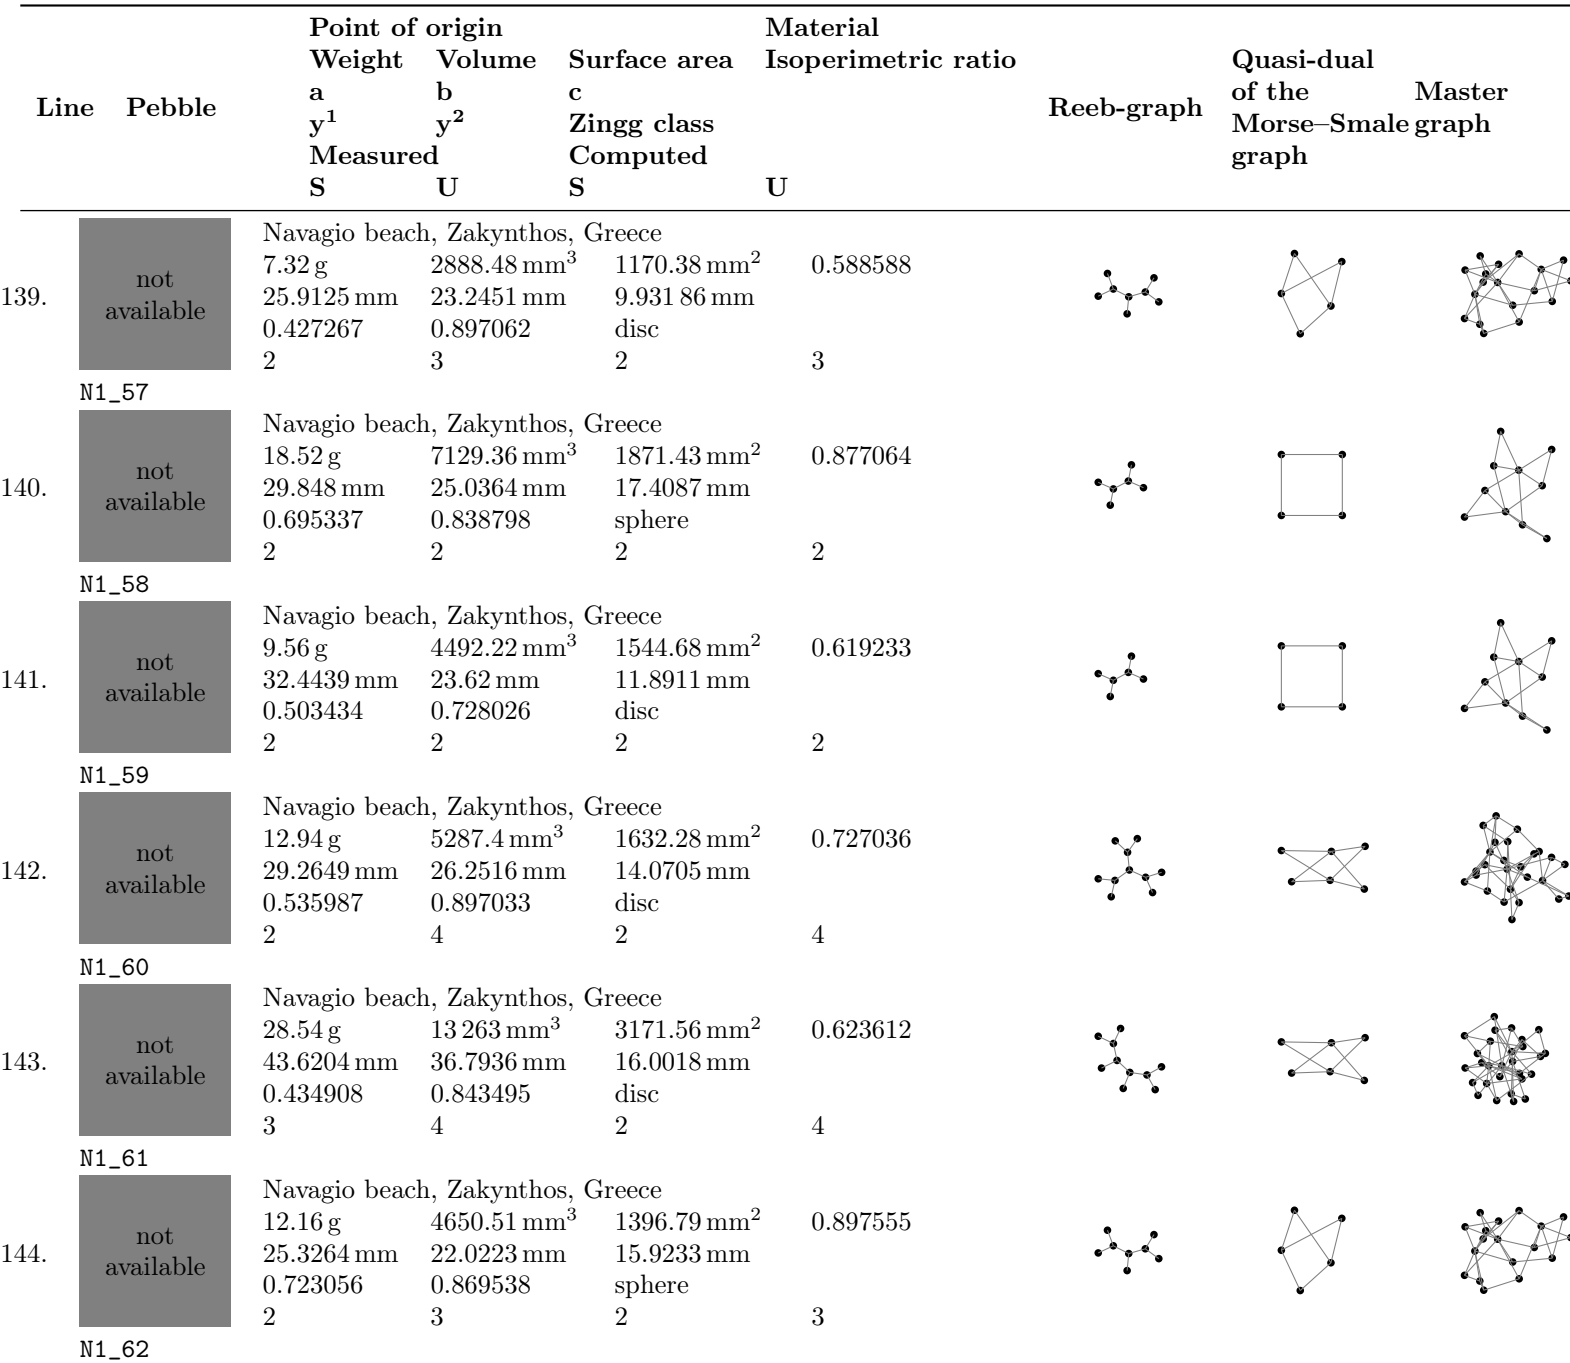 | 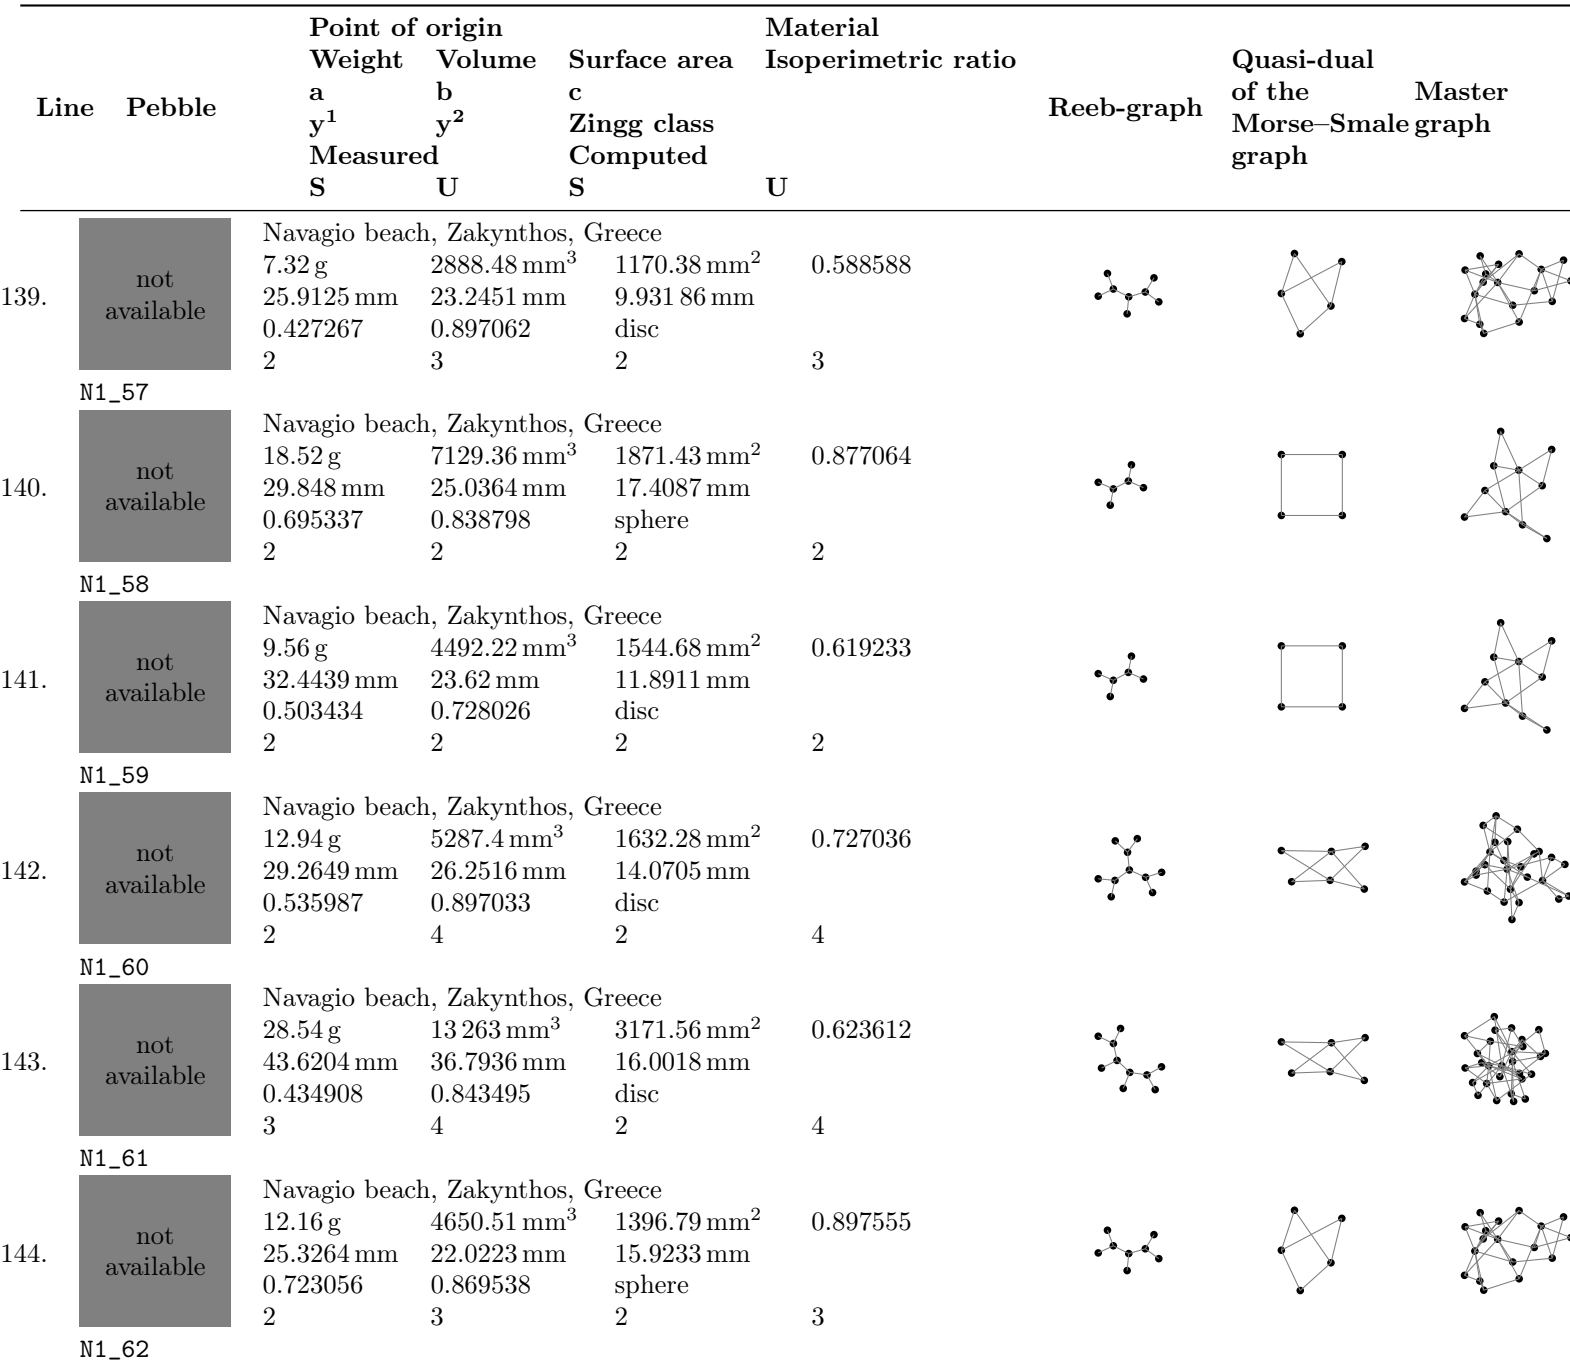 | 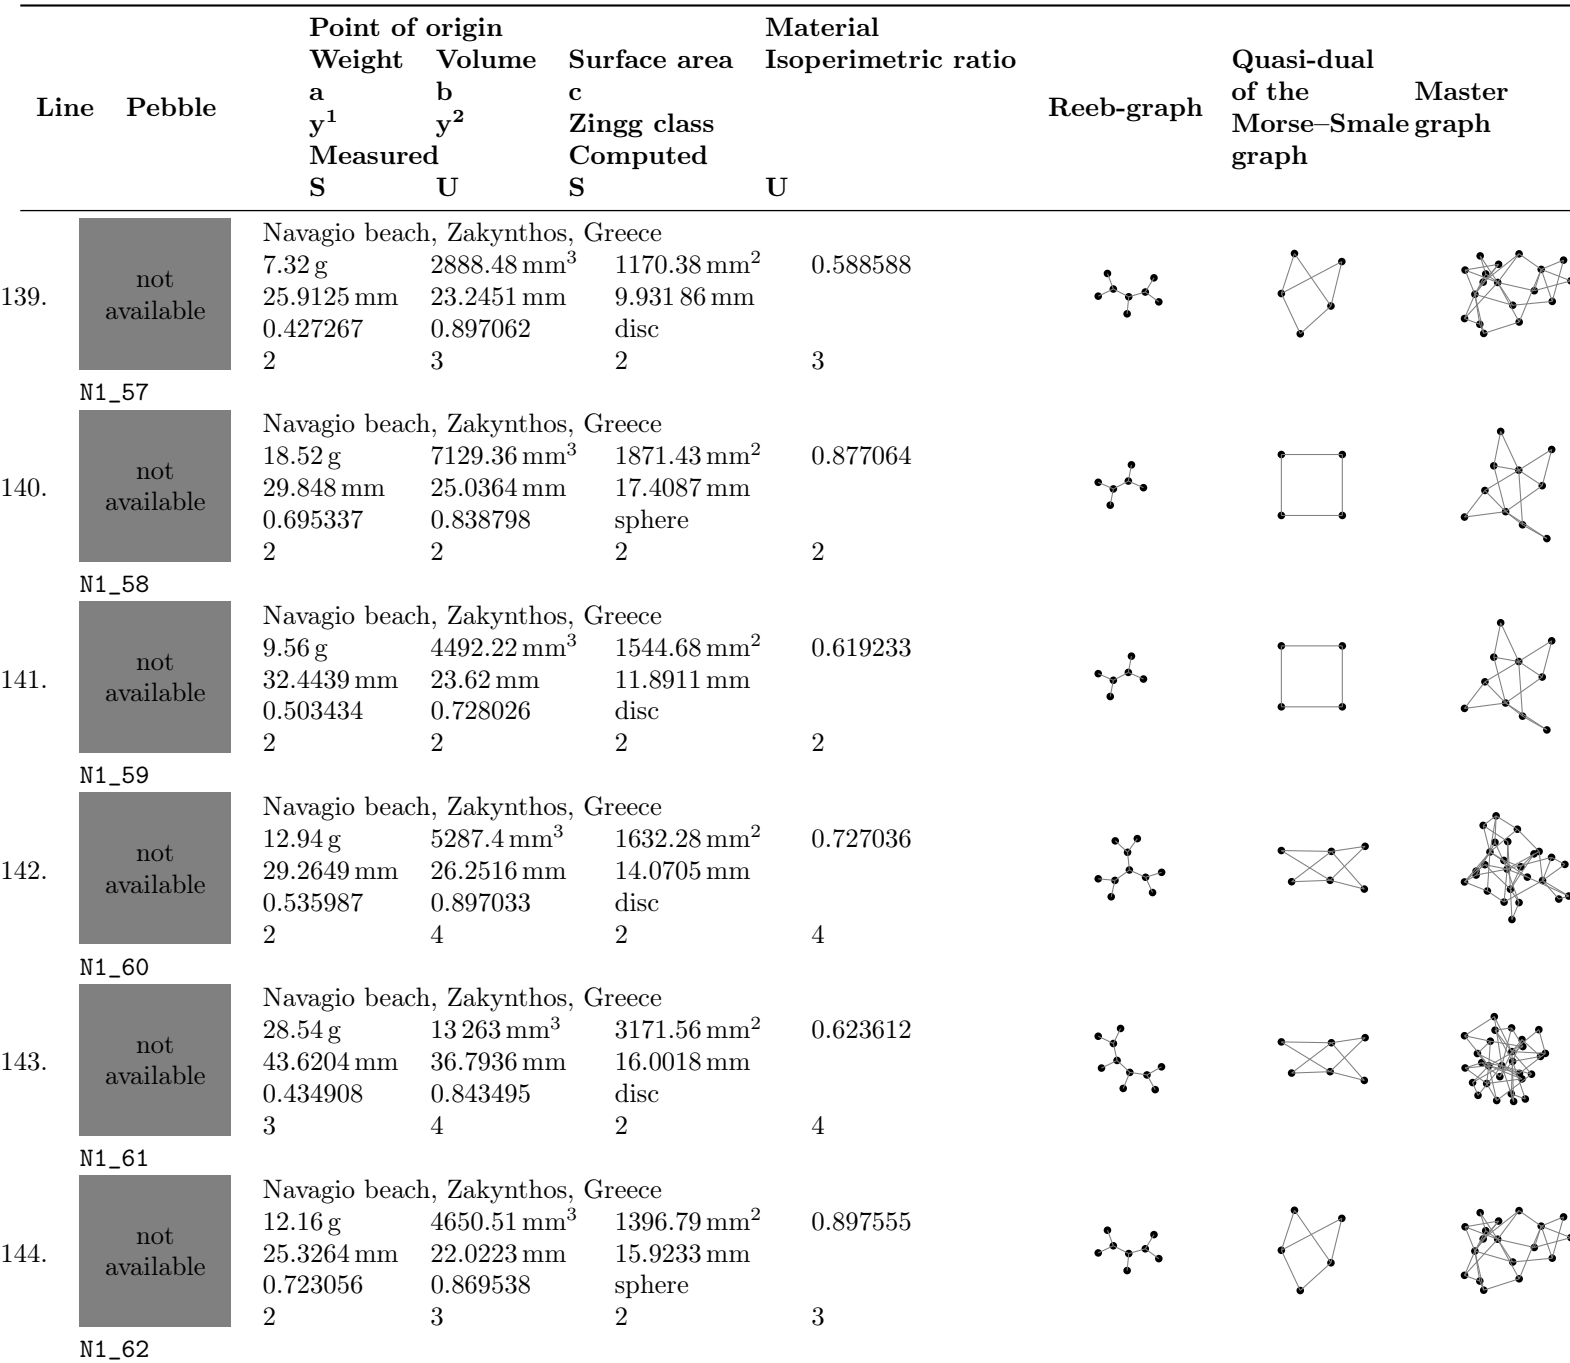 |
|      |                               | 12.16 g                          | 4650.51 mm <sup>3</sup> | 1396.79 mm <sup>2</sup>      |                                      |                                                                                       |                                                                                       |                                                                                       |
|      |                               | 25.3264 mm                       | 22.0223 mm              | 15.9233 mm                   |                                      |                                                                                       |                                                                                       |                                                                                       |
|      |                               | 0.723056                         | 0.869538                | sphere                       |                                      |                                                                                       |                                                                                       |                                                                                       |
|      |                               | 2                                | 3                       | 2                            |                                      |                                                                                       |                                                                                       |                                                                                       |
|      |                               |                                  |                         |                              |                                      |                                                                                       |                                                                                       |                                                                                       |

| Line  | Pebble                                                                              | Point of origin                      |                          | Surface area<br>c<br>Zingg class<br>Computed<br>S | Material<br>Isoperimetric ratio<br>U | Reeb-graph                                                                            | Quasi-dual<br>of the<br>Morse–Smale<br>graph                                          | Master<br>graph                                                                       |
|-------|-------------------------------------------------------------------------------------|--------------------------------------|--------------------------|---------------------------------------------------|--------------------------------------|---------------------------------------------------------------------------------------|---------------------------------------------------------------------------------------|---------------------------------------------------------------------------------------|
|       |                                                                                     | Weight                               | Volume                   |                                                   |                                      |                                                                                       |                                                                                       |                                                                                       |
|       |                                                                                     | a<br>y <sup>1</sup><br>Measured<br>S | b<br>y <sup>2</sup><br>U |                                                   |                                      |                                                                                       |                                                                                       |                                                                                       |
|       |                                                                                     |                                      |                          |                                                   |                                      |                                                                                       |                                                                                       |                                                                                       |
| 145.  | 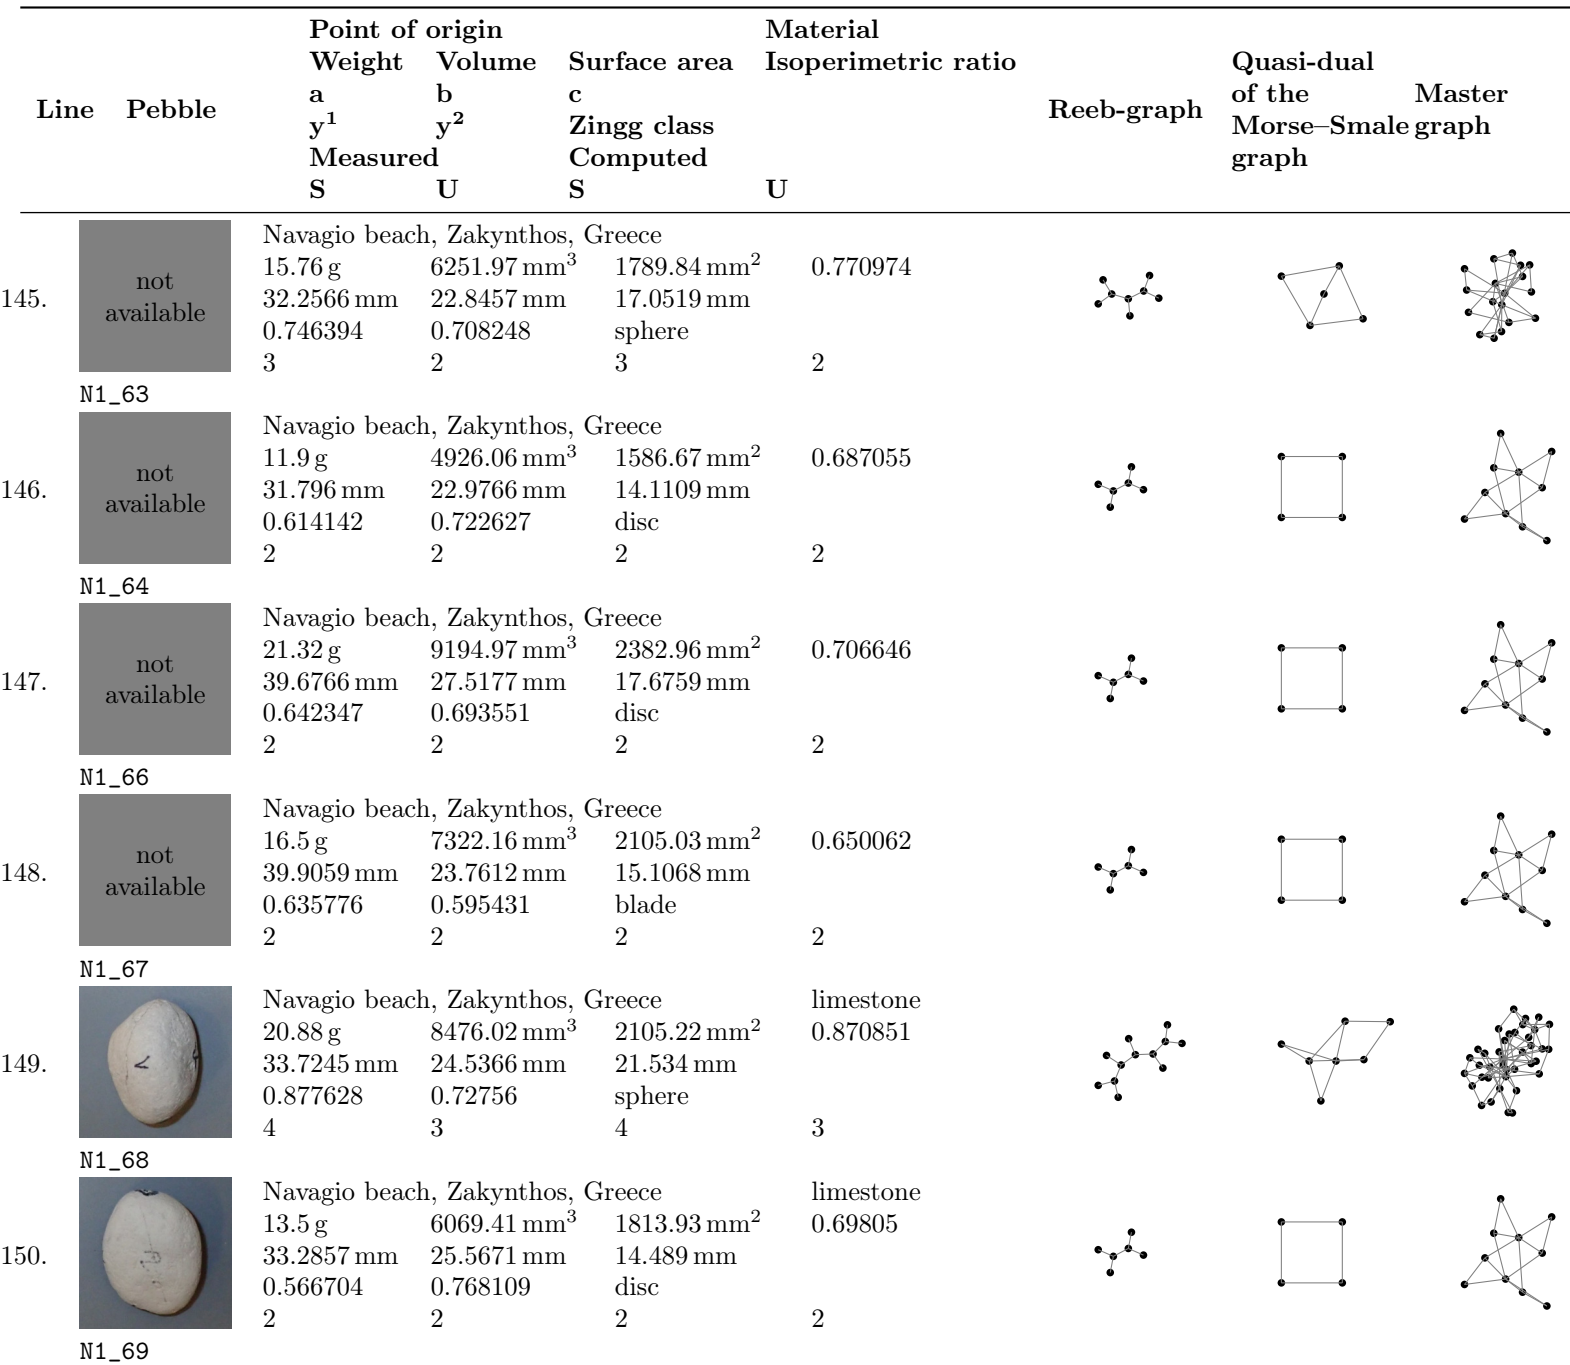   | Navagio beach, Zakynthos, Greece     |                          |                                                   | 0.770974                             | 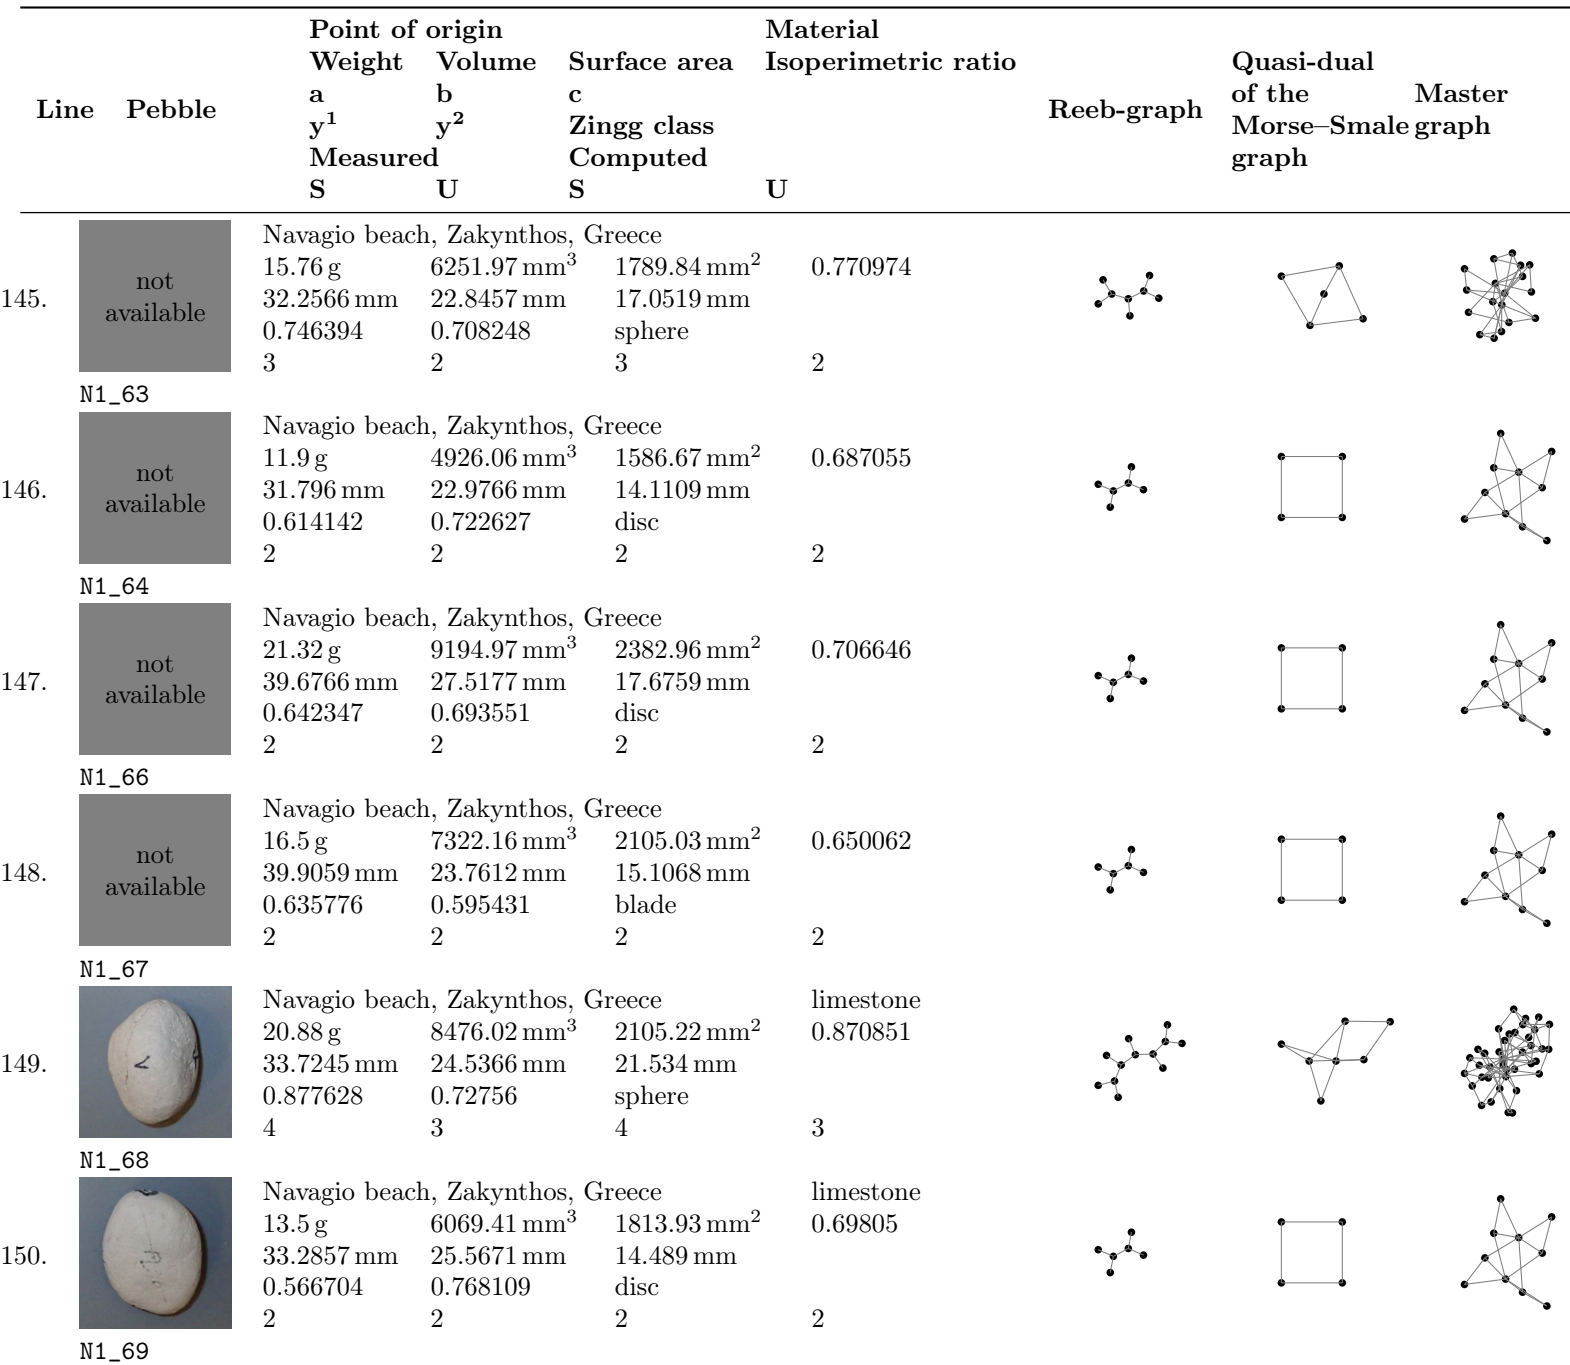   | 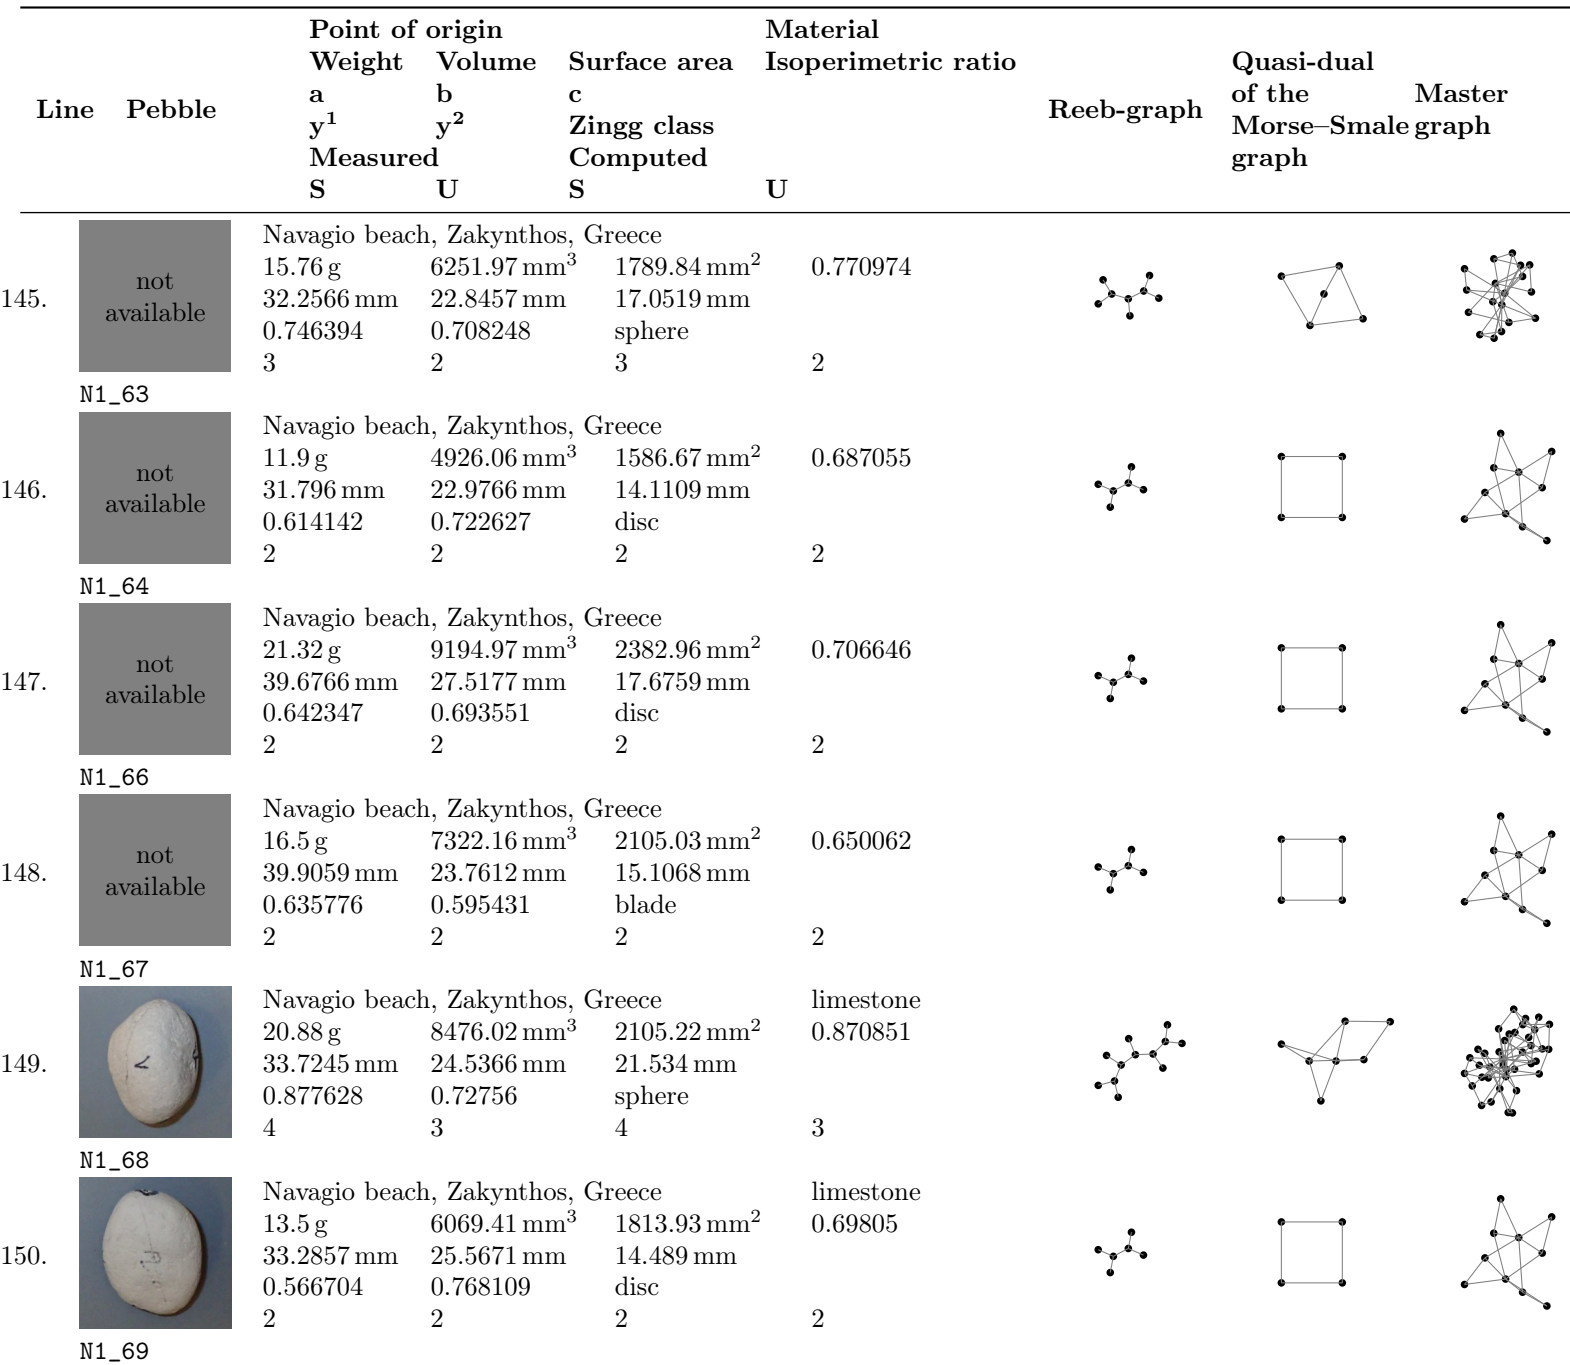   | 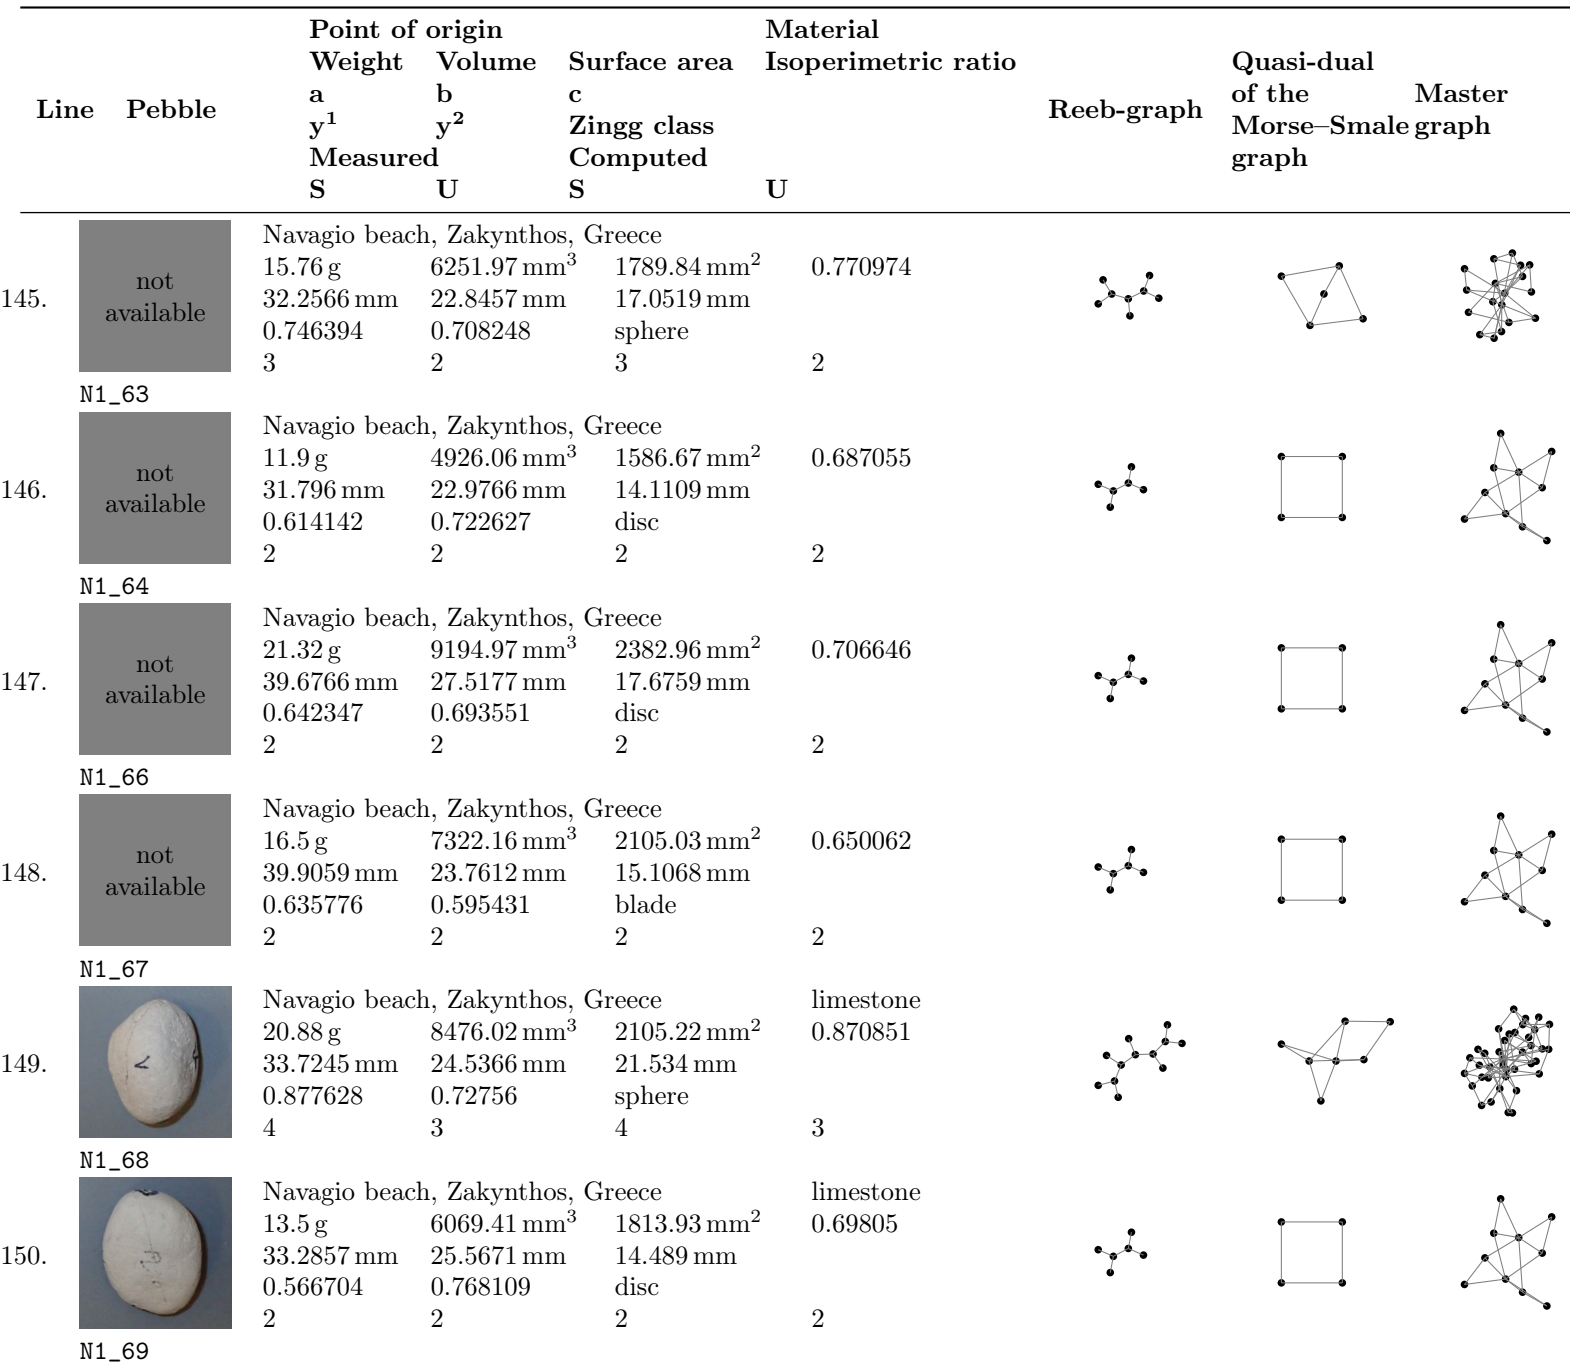   |
|       |                                                                                     | 15.76 g                              | 6251.97 mm <sup>3</sup>  | 1789.84 mm <sup>2</sup>                           |                                      |                                                                                       |                                                                                       |                                                                                       |
|       |                                                                                     | 32.2566 mm                           | 22.8457 mm               | 17.0519 mm                                        |                                      |                                                                                       |                                                                                       |                                                                                       |
|       |                                                                                     | 0.746394                             | 0.708248                 | sphere                                            |                                      |                                                                                       |                                                                                       |                                                                                       |
|       |                                                                                     | 3                                    | 2                        | 3                                                 |                                      |                                                                                       |                                                                                       |                                                                                       |
| N1_63 |                                                                                     |                                      |                          |                                                   |                                      |                                                                                       |                                                                                       |                                                                                       |
| 146.  | 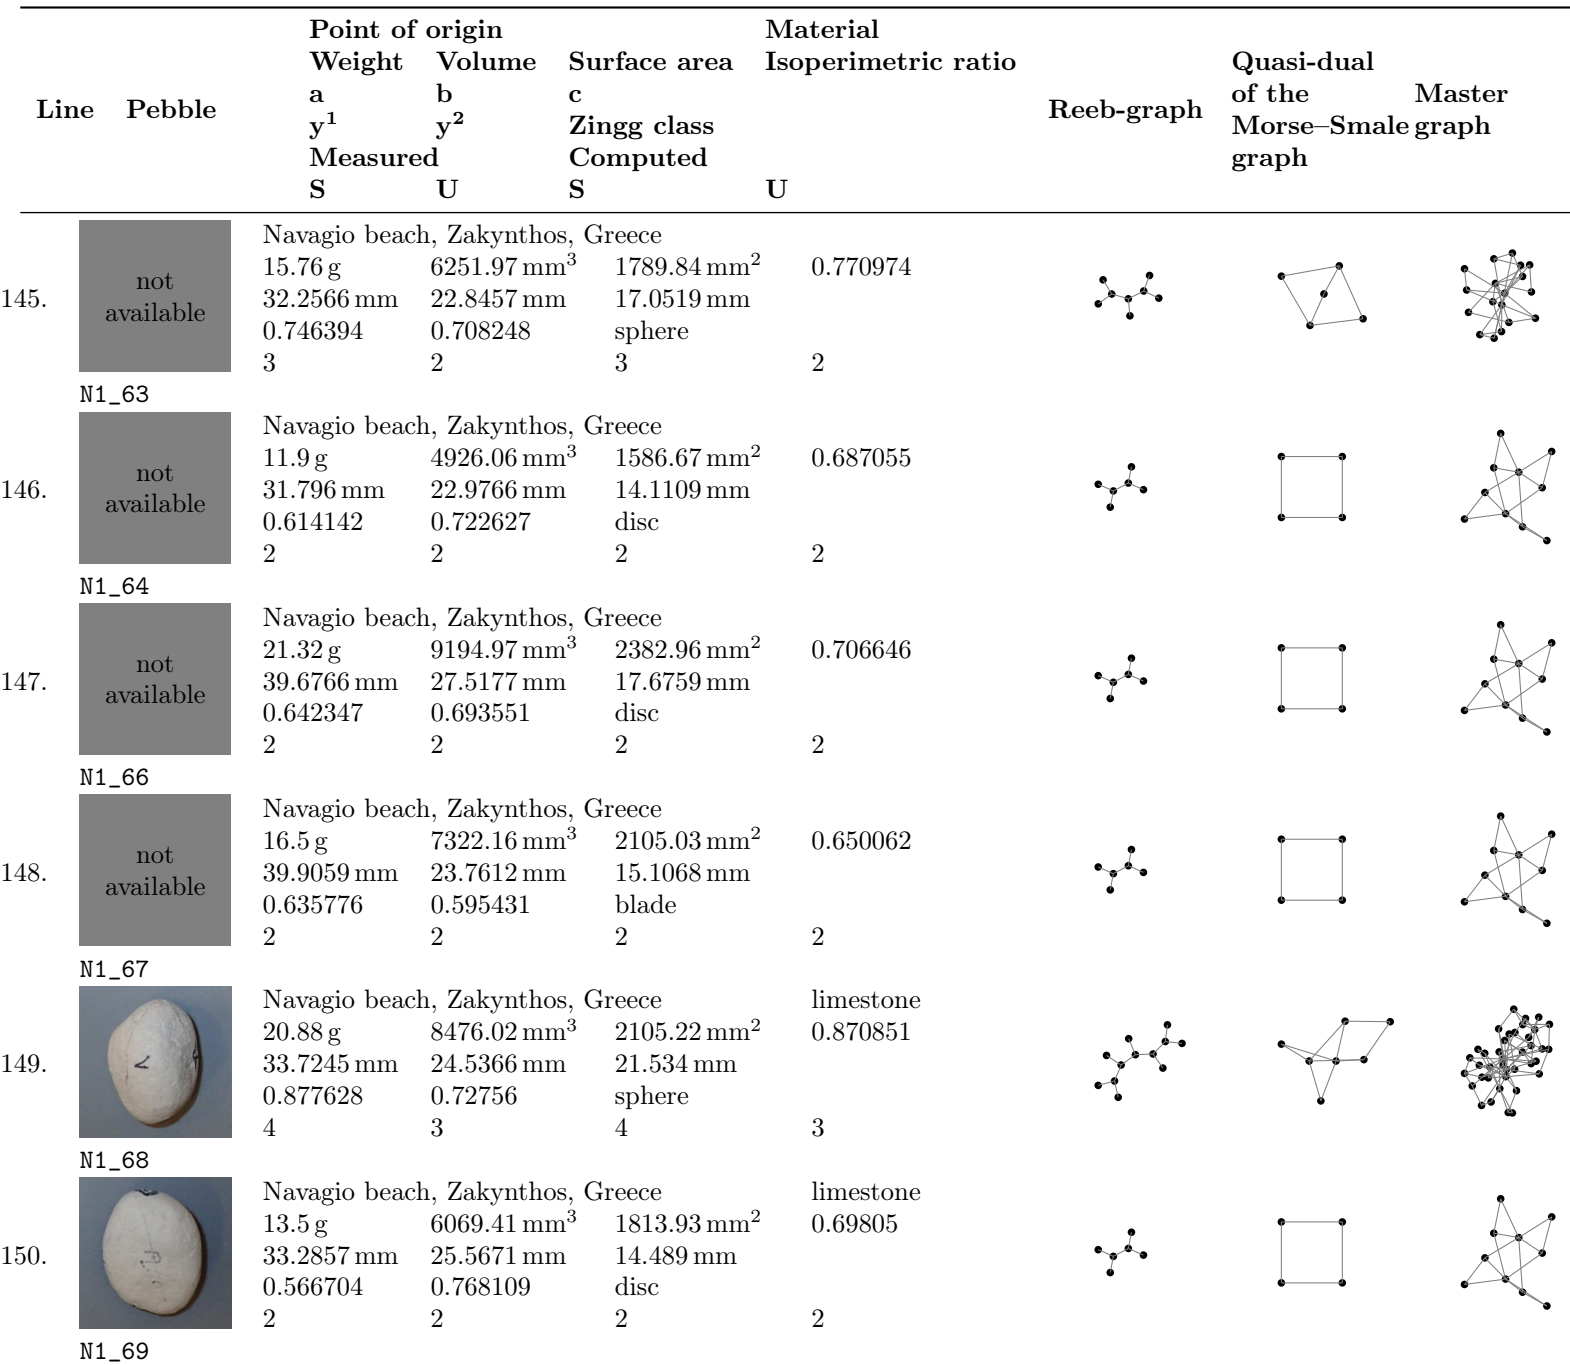   | Navagio beach, Zakynthos, Greece     |                          |                                                   | 0.687055                             | 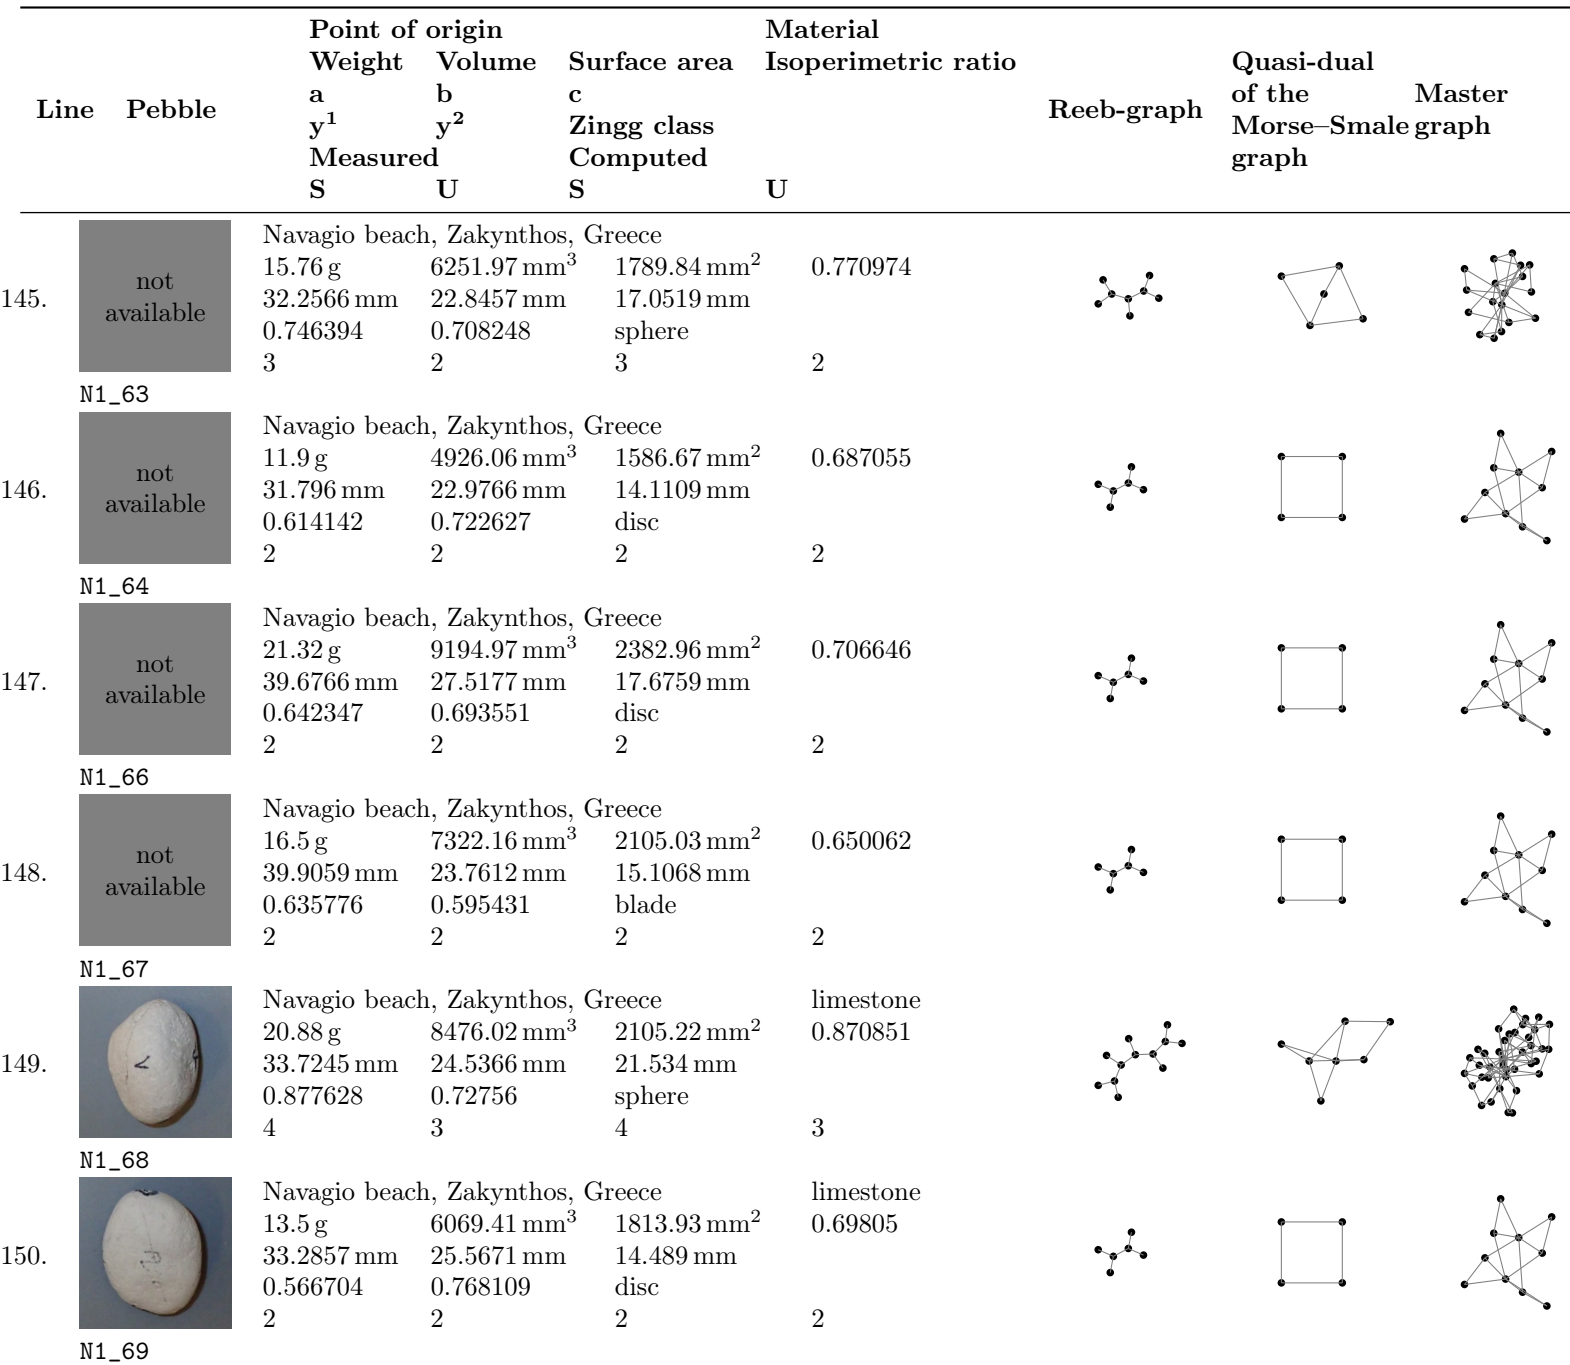   | 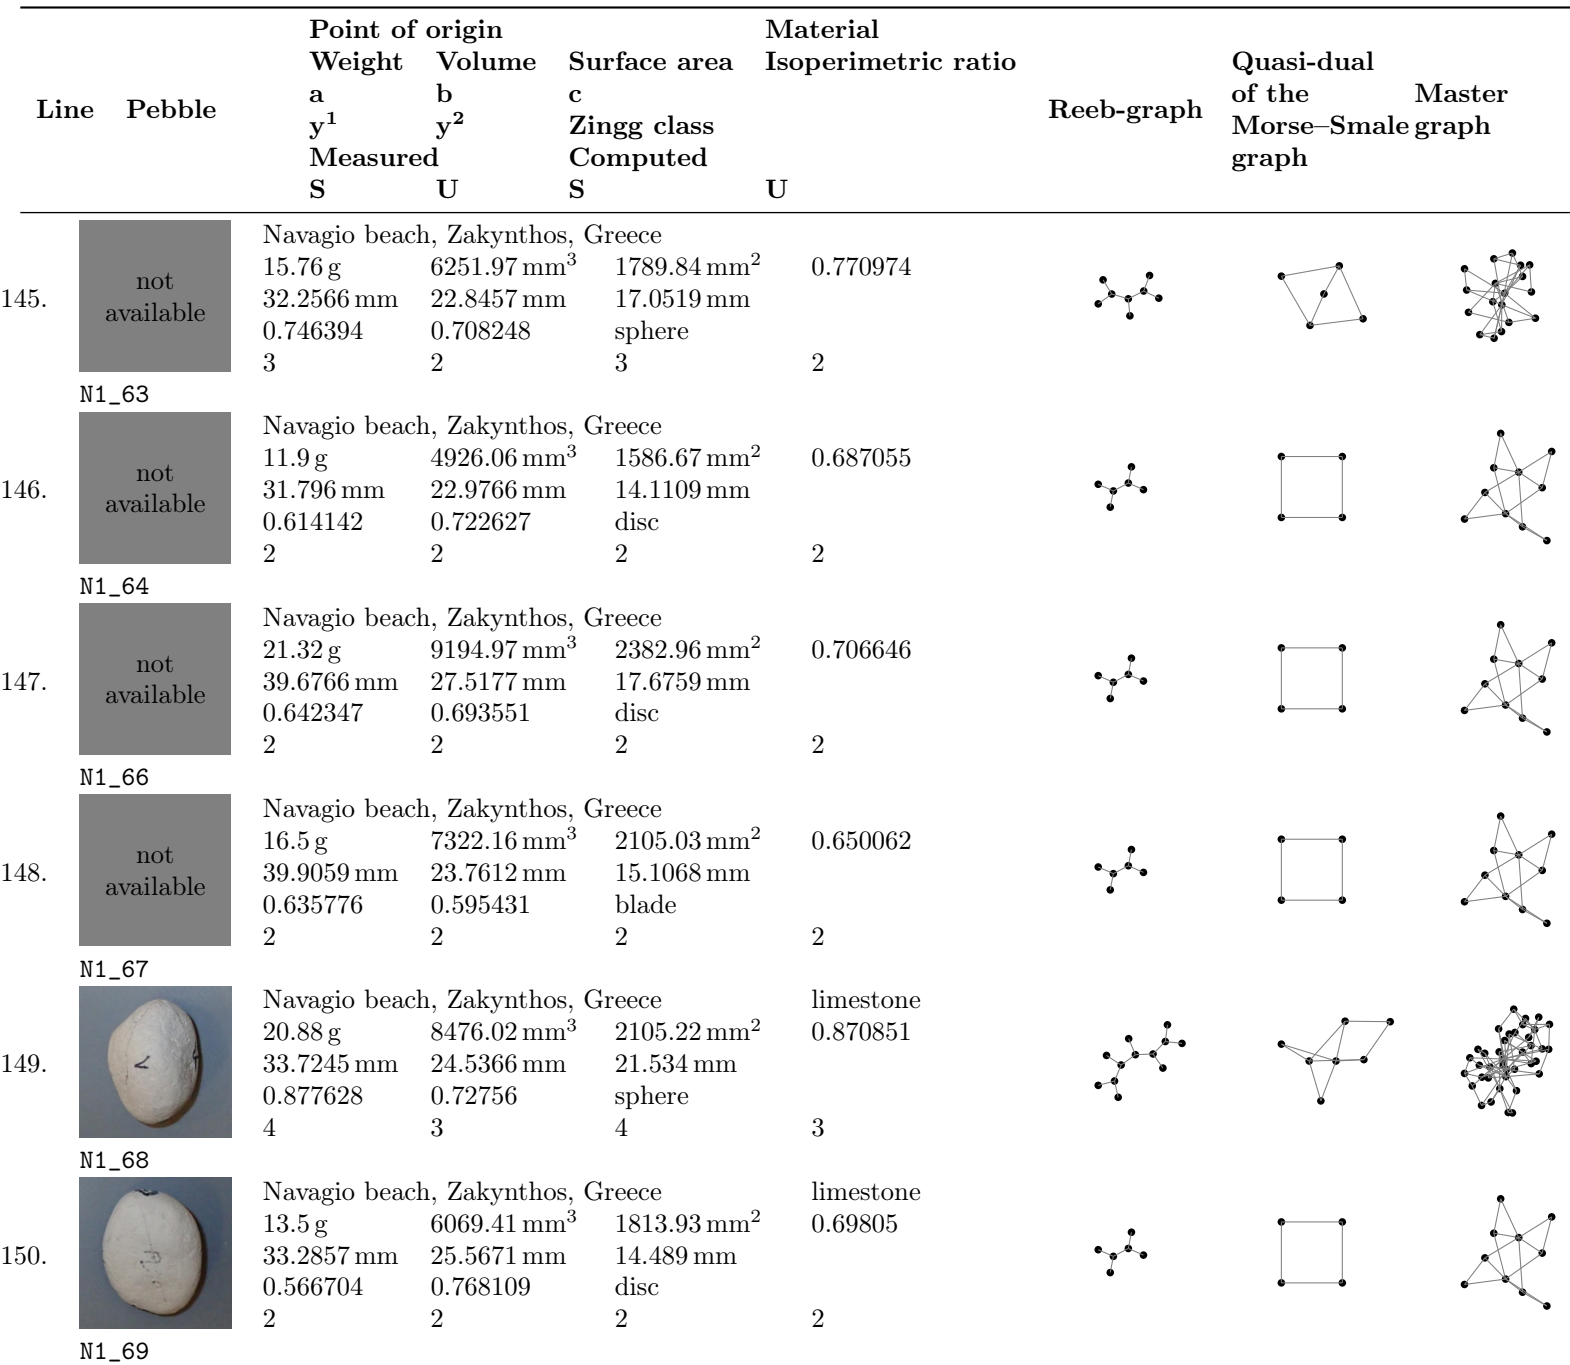   | 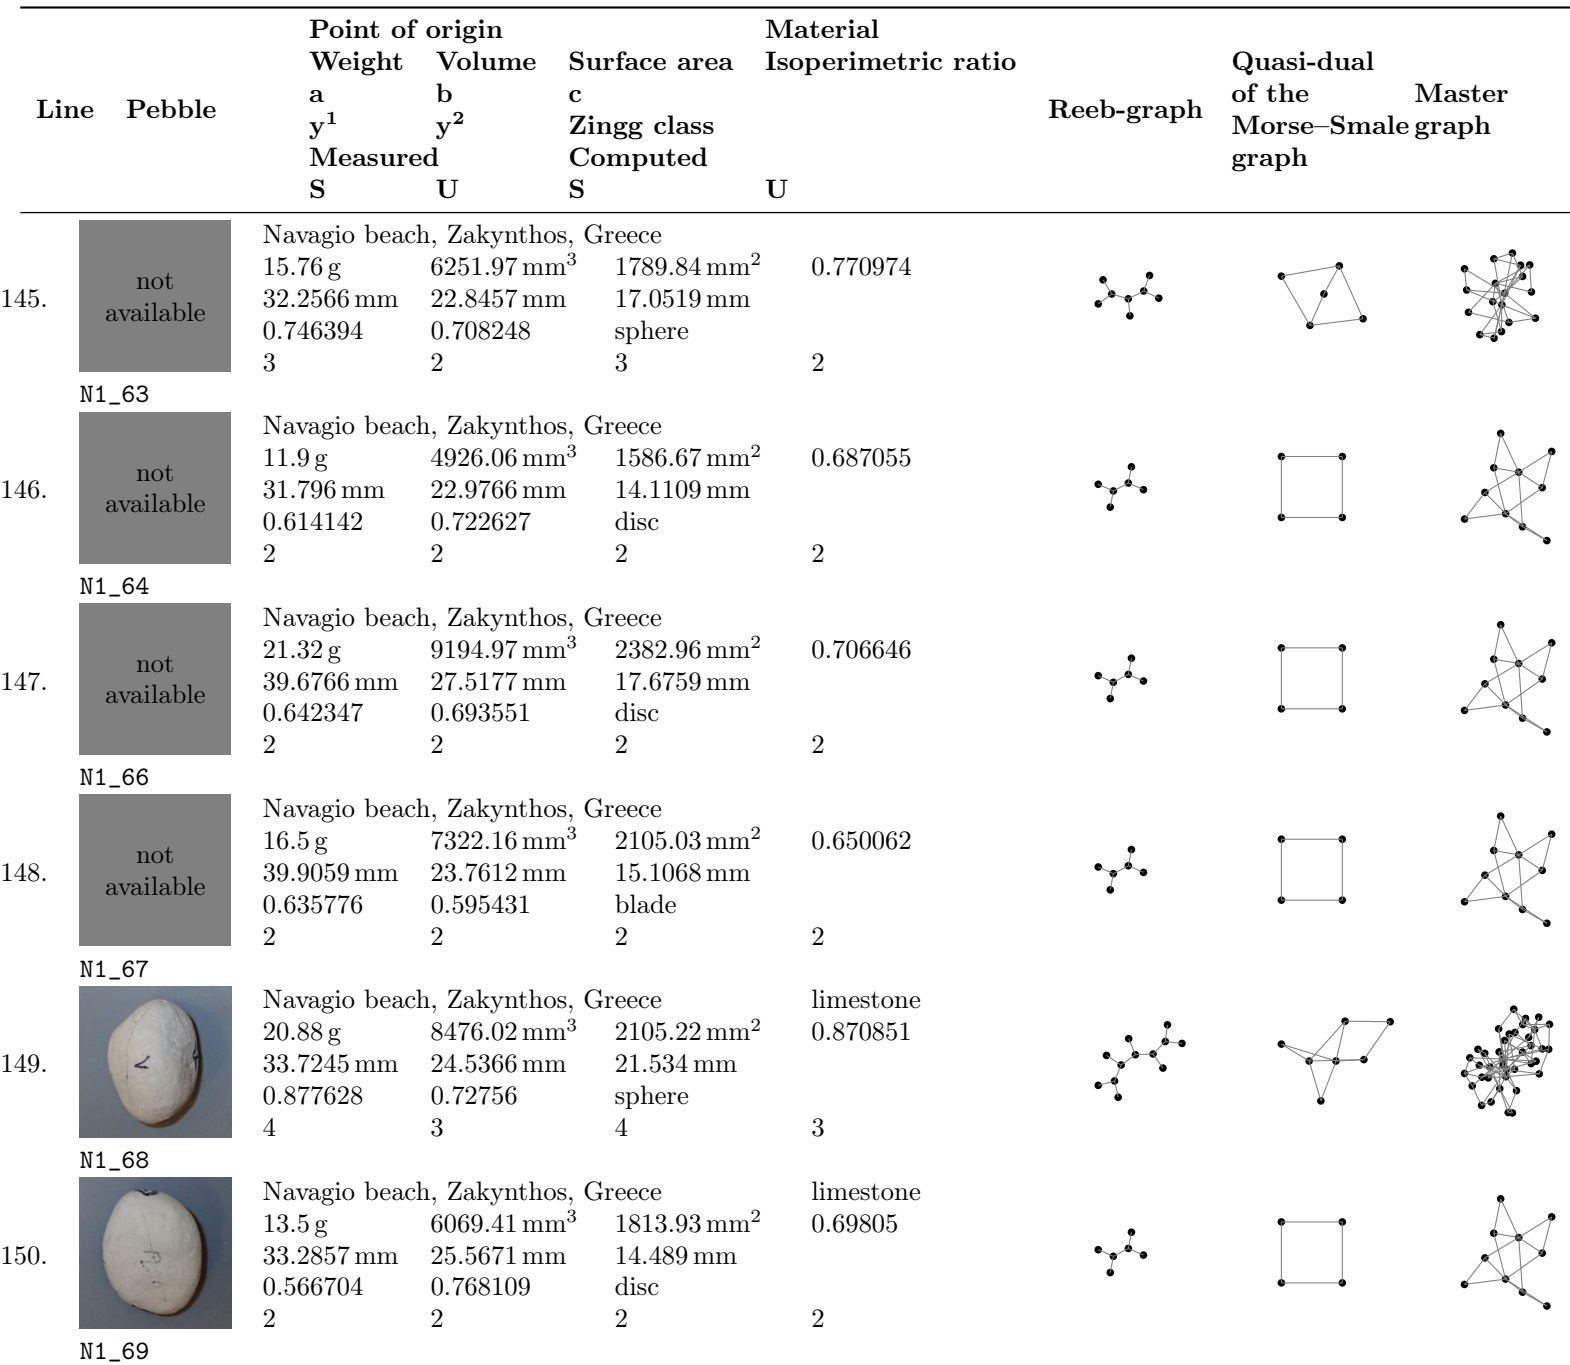   |
|       |                                                                                     | 11.9 g                               | 4926.06 mm <sup>3</sup>  | 1586.67 mm <sup>2</sup>                           |                                      |                                                                                       |                                                                                       |                                                                                       |
|       |                                                                                     | 31.796 mm                            | 22.9766 mm               | 14.1109 mm                                        |                                      |                                                                                       |                                                                                       |                                                                                       |
|       |                                                                                     | 0.614142                             | 0.722627                 | disc                                              |                                      |                                                                                       |                                                                                       |                                                                                       |
|       |                                                                                     | 2                                    | 2                        | 2                                                 |                                      |                                                                                       |                                                                                       |                                                                                       |
| N1_64 |                                                                                     |                                      |                          |                                                   |                                      |                                                                                       |                                                                                       |                                                                                       |
| 147.  | 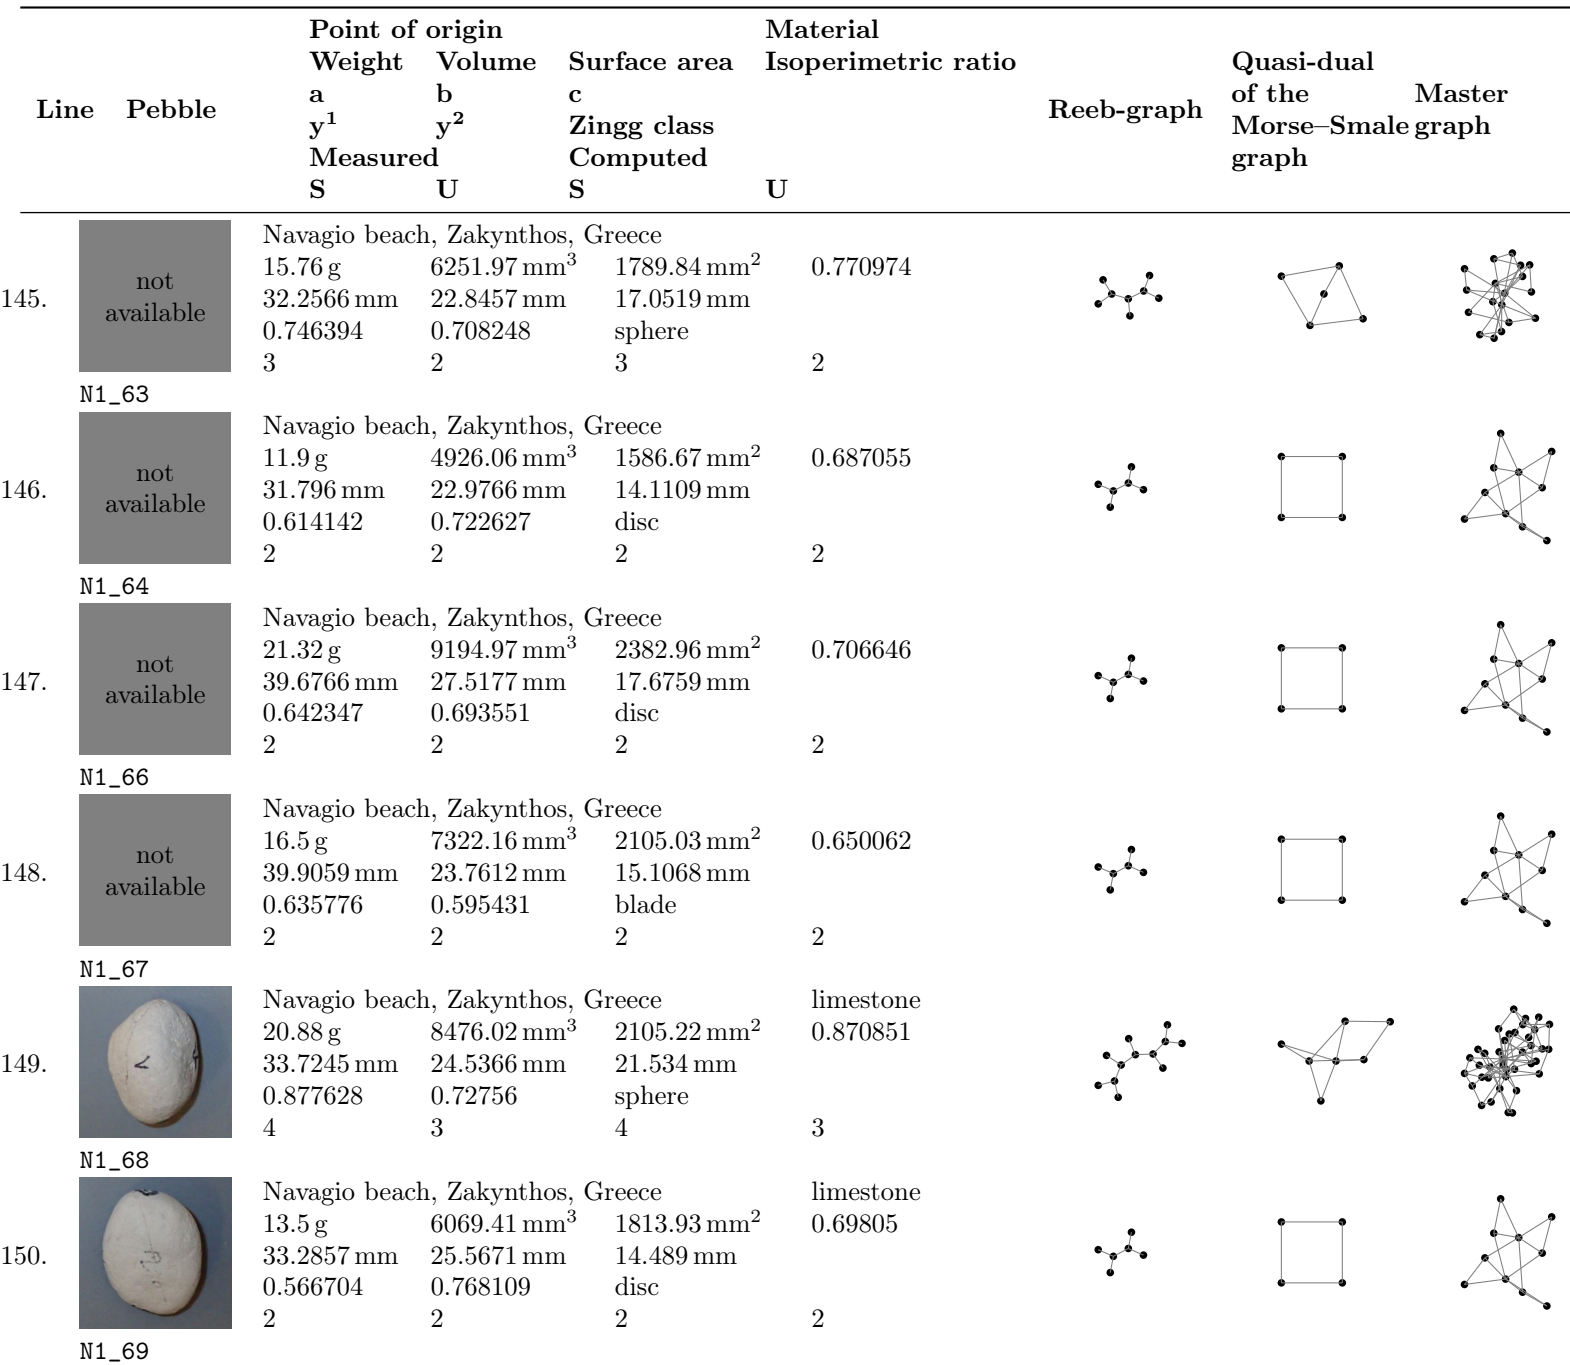   | Navagio beach, Zakynthos, Greece     |                          |                                                   | 0.706646                             | 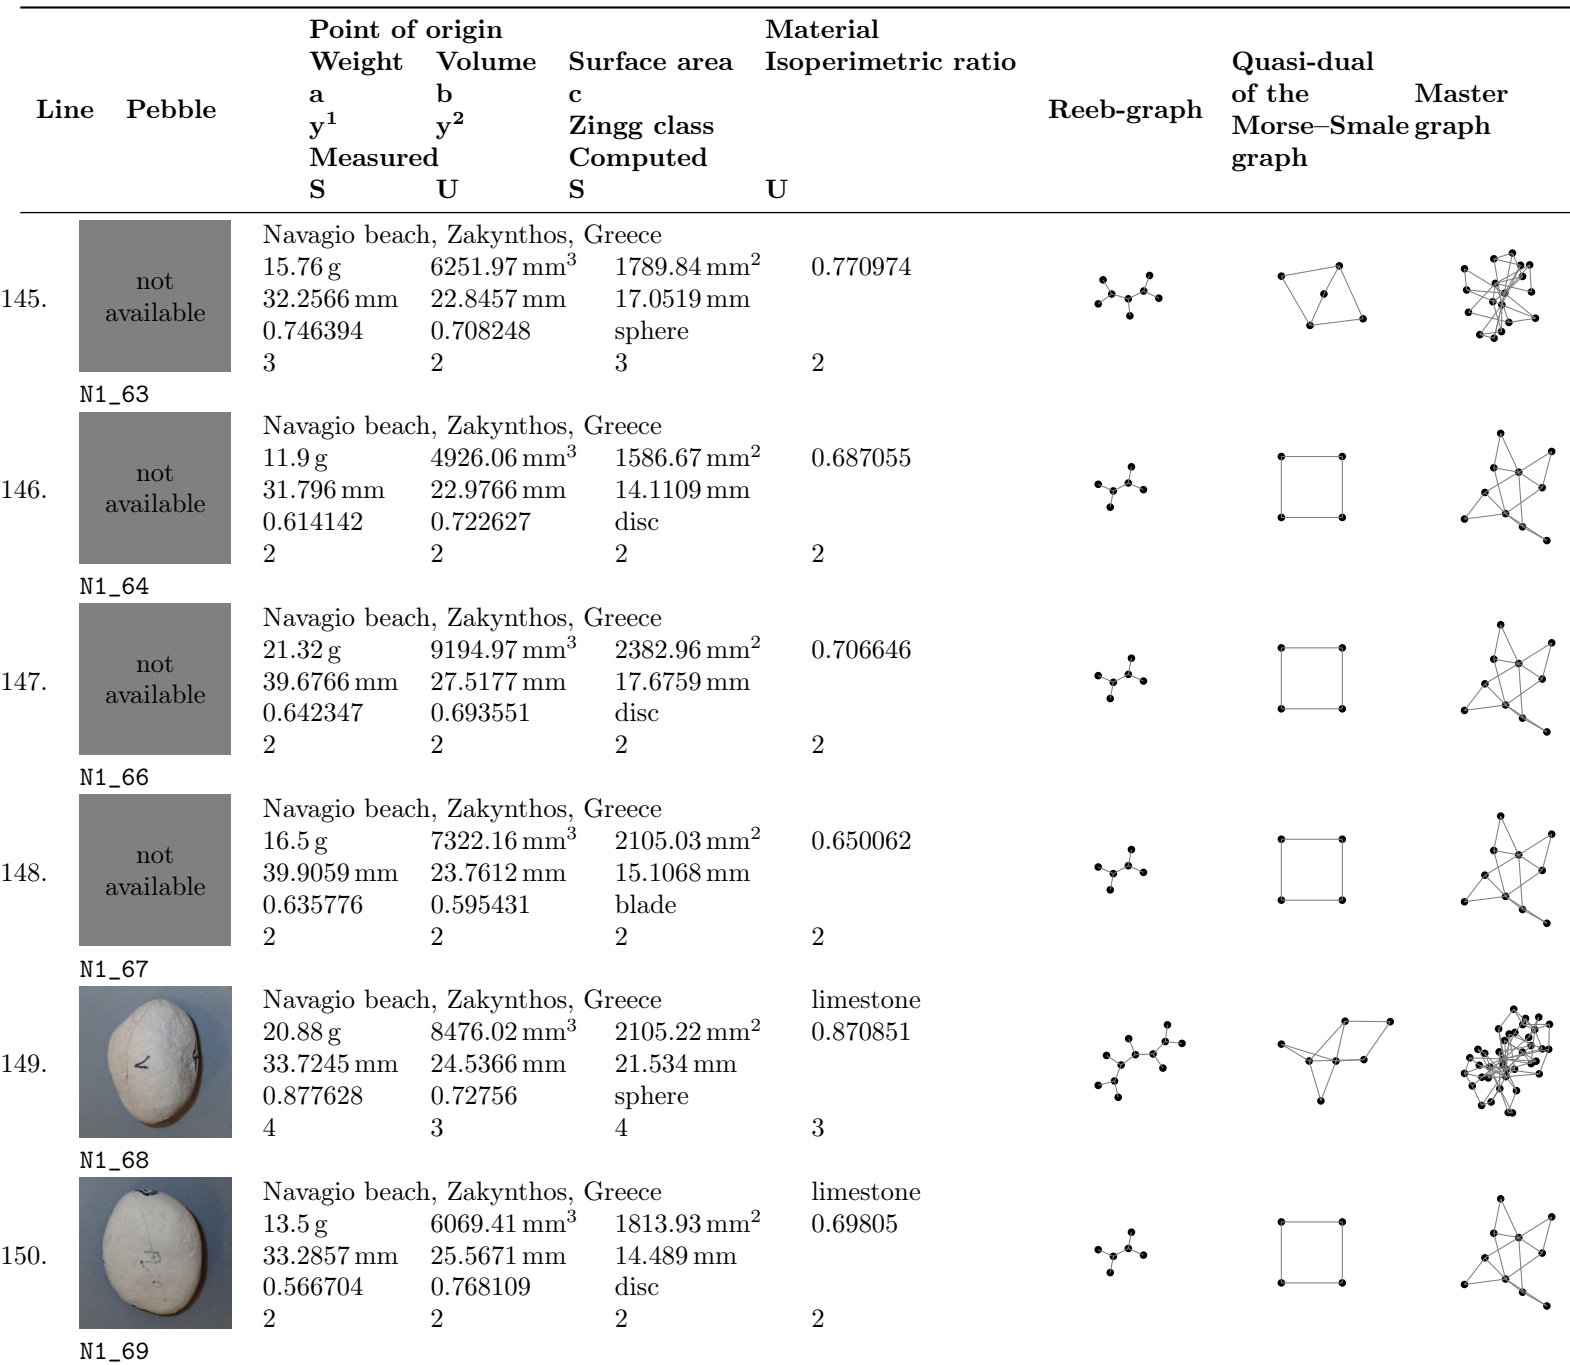   | 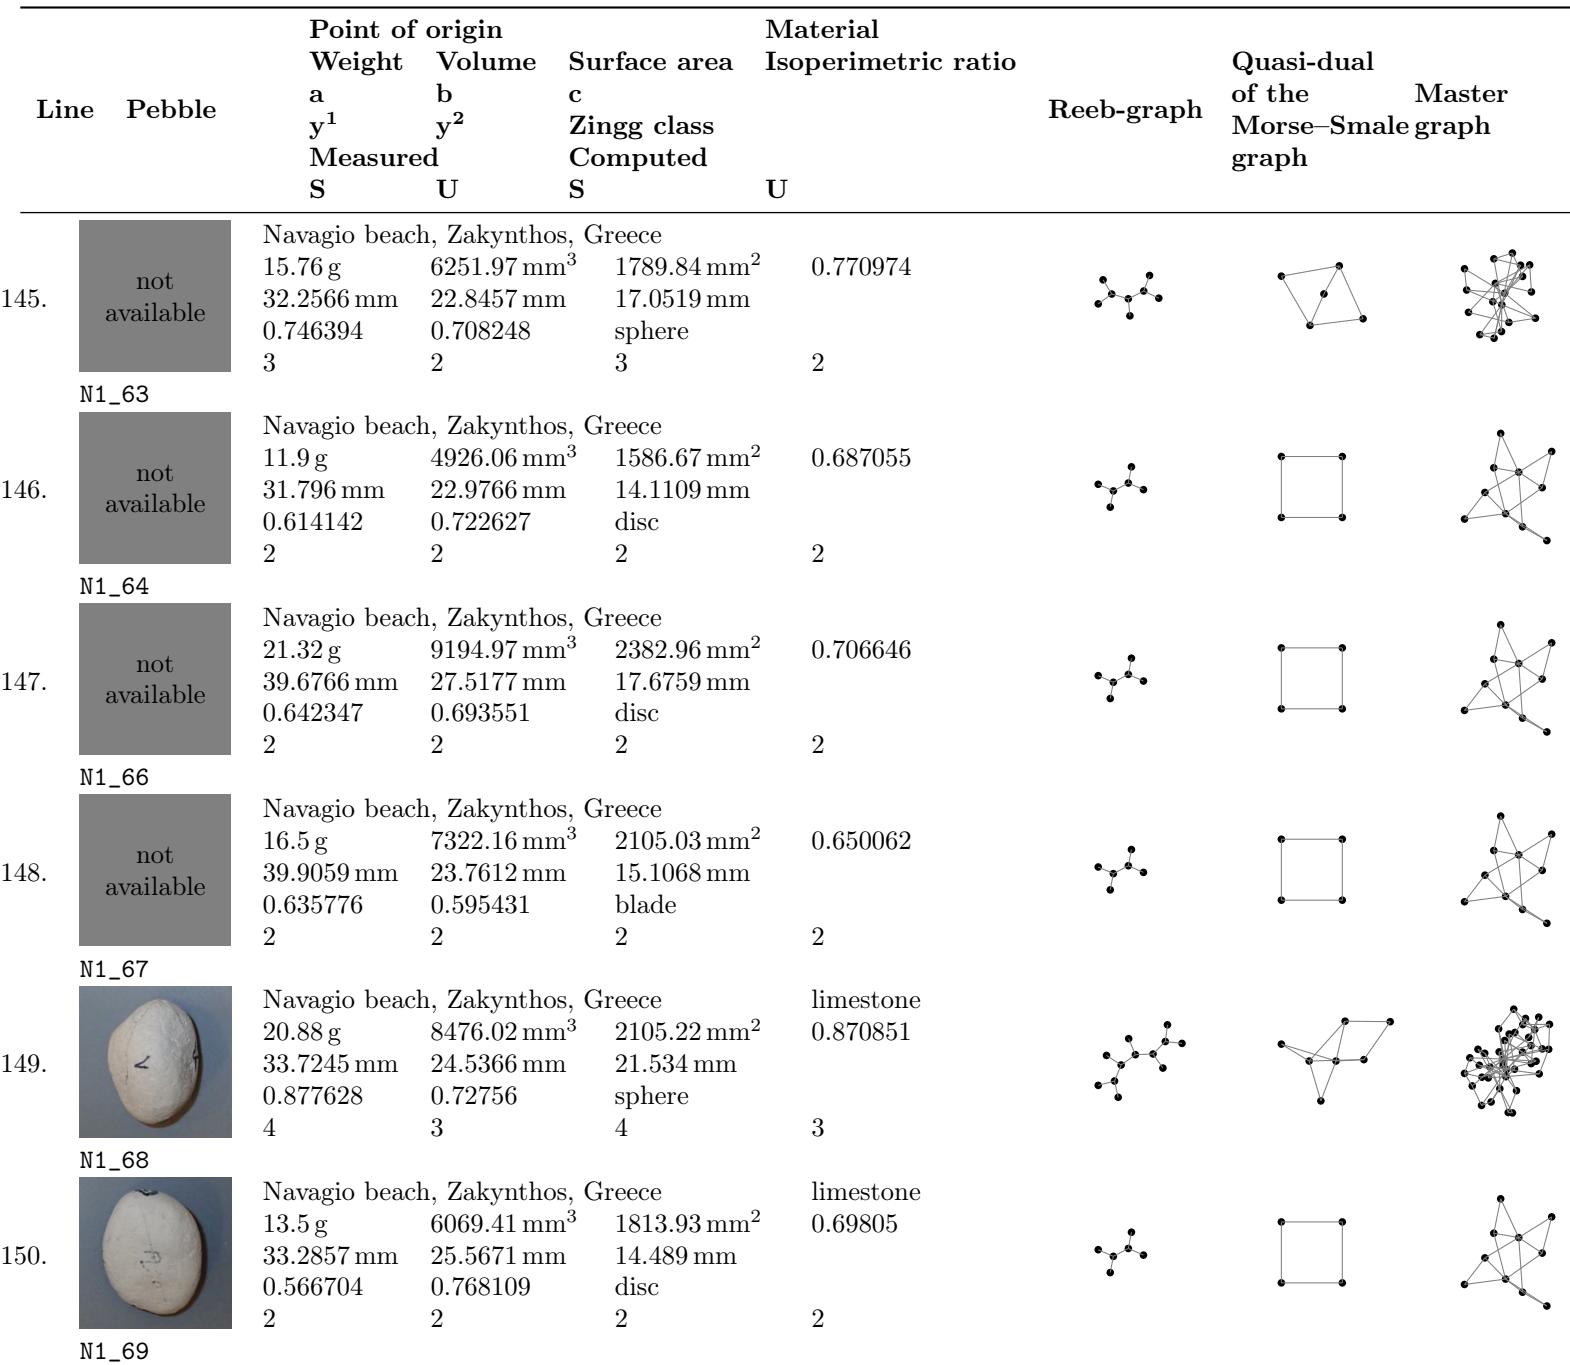   | 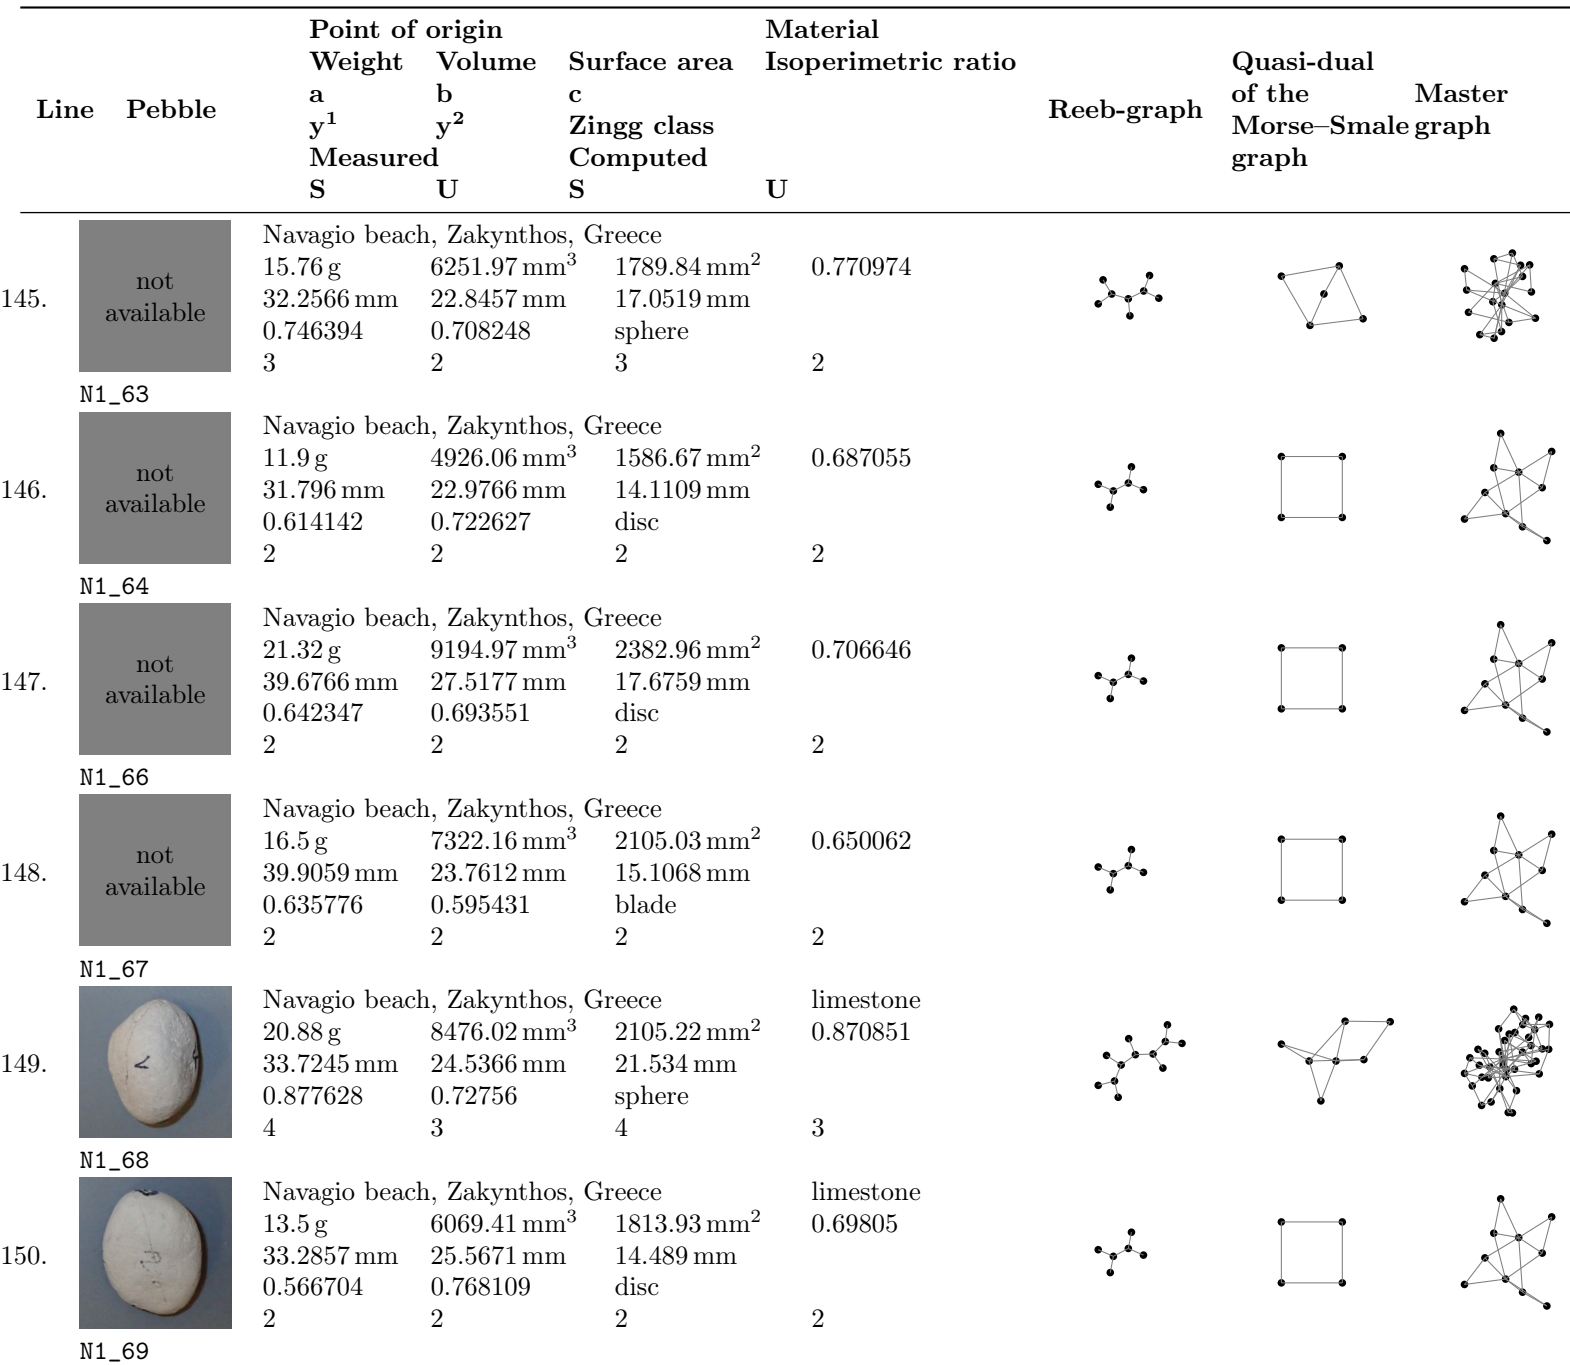   |
|       |                                                                                     | 21.32 g                              | 9194.97 mm <sup>3</sup>  | 2382.96 mm <sup>2</sup>                           |                                      |                                                                                       |                                                                                       |                                                                                       |
|       |                                                                                     | 39.6766 mm                           | 27.5177 mm               | 17.6759 mm                                        |                                      |                                                                                       |                                                                                       |                                                                                       |
|       |                                                                                     | 0.642347                             | 0.693551                 | disc                                              |                                      |                                                                                       |                                                                                       |                                                                                       |
|       |                                                                                     | 2                                    | 2                        | 2                                                 |                                      |                                                                                       |                                                                                       |                                                                                       |
| N1_66 |                                                                                     |                                      |                          |                                                   |                                      |                                                                                       |                                                                                       |                                                                                       |
| 148.  | 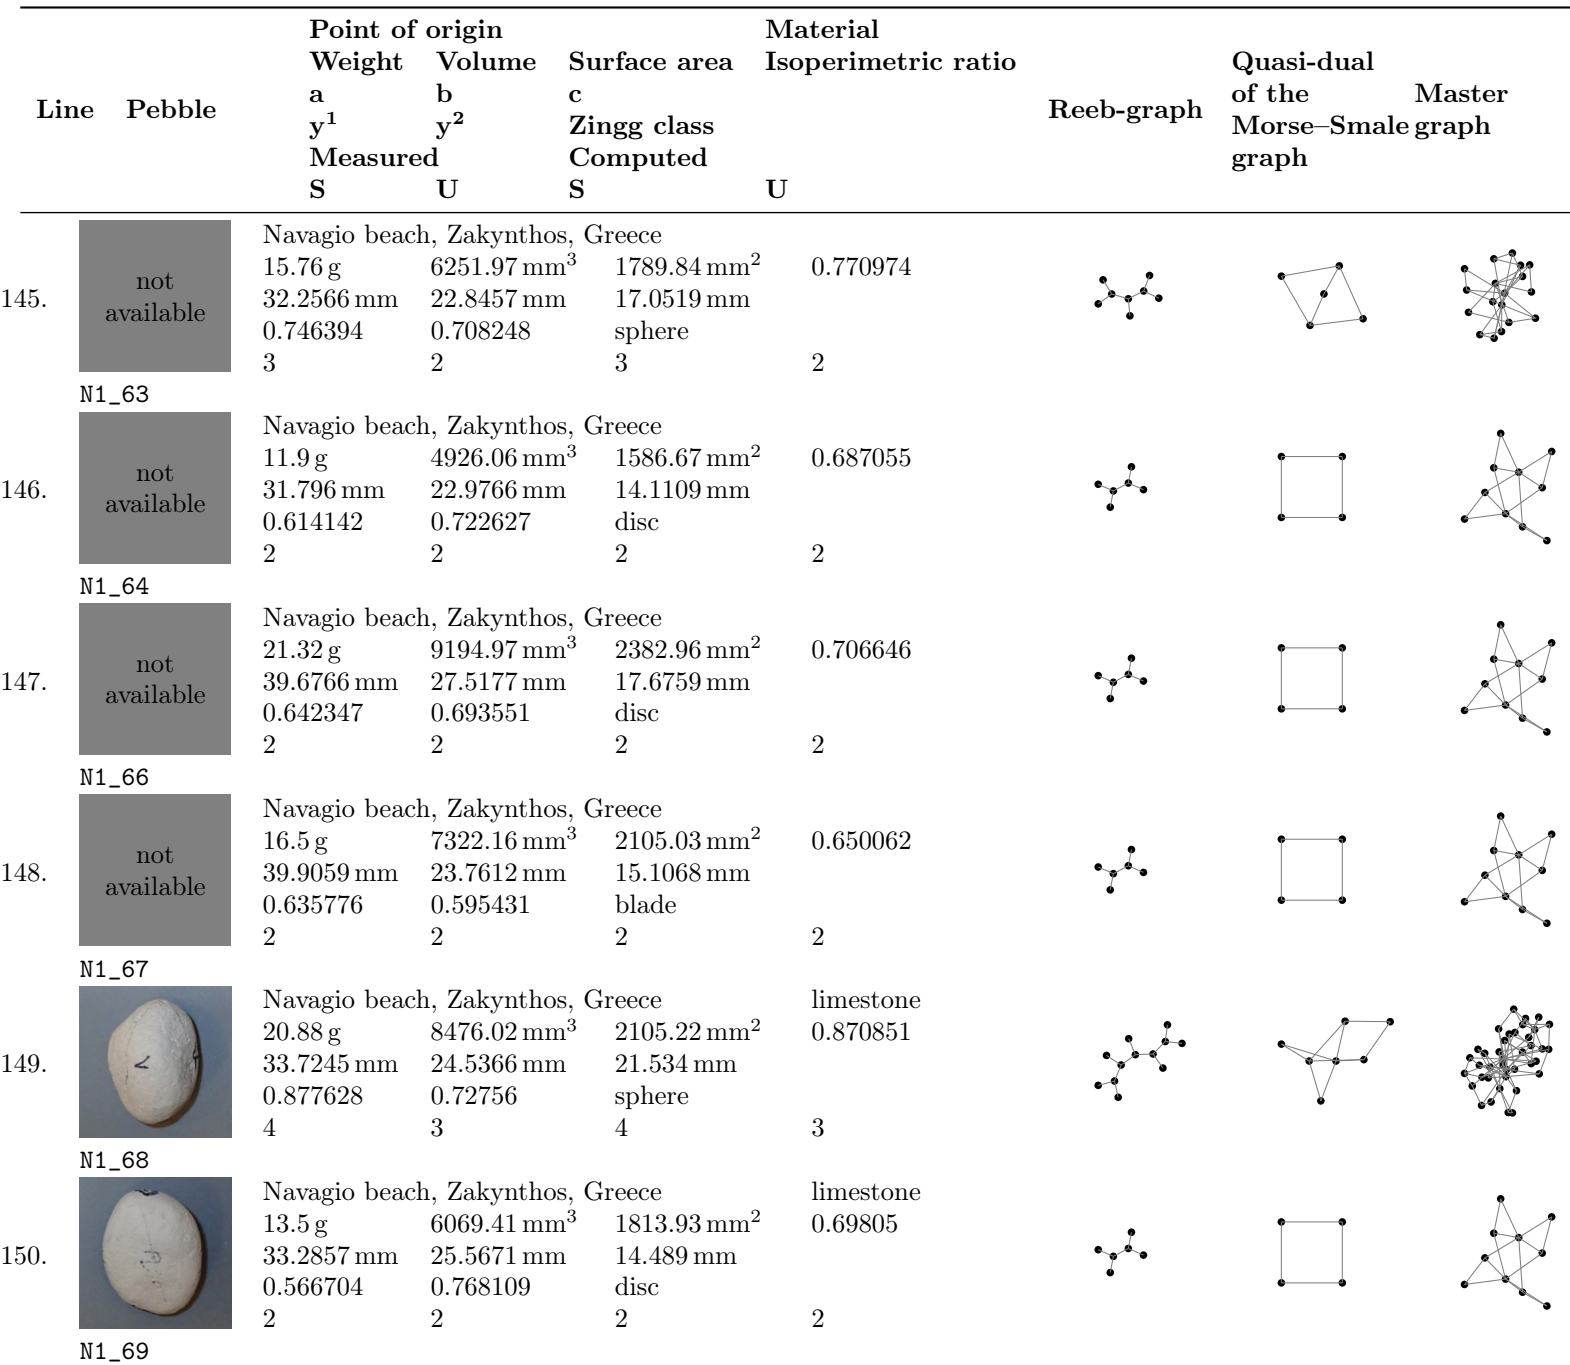  | Navagio beach, Zakynthos, Greece     |                          |                                                   | 0.650062                             | 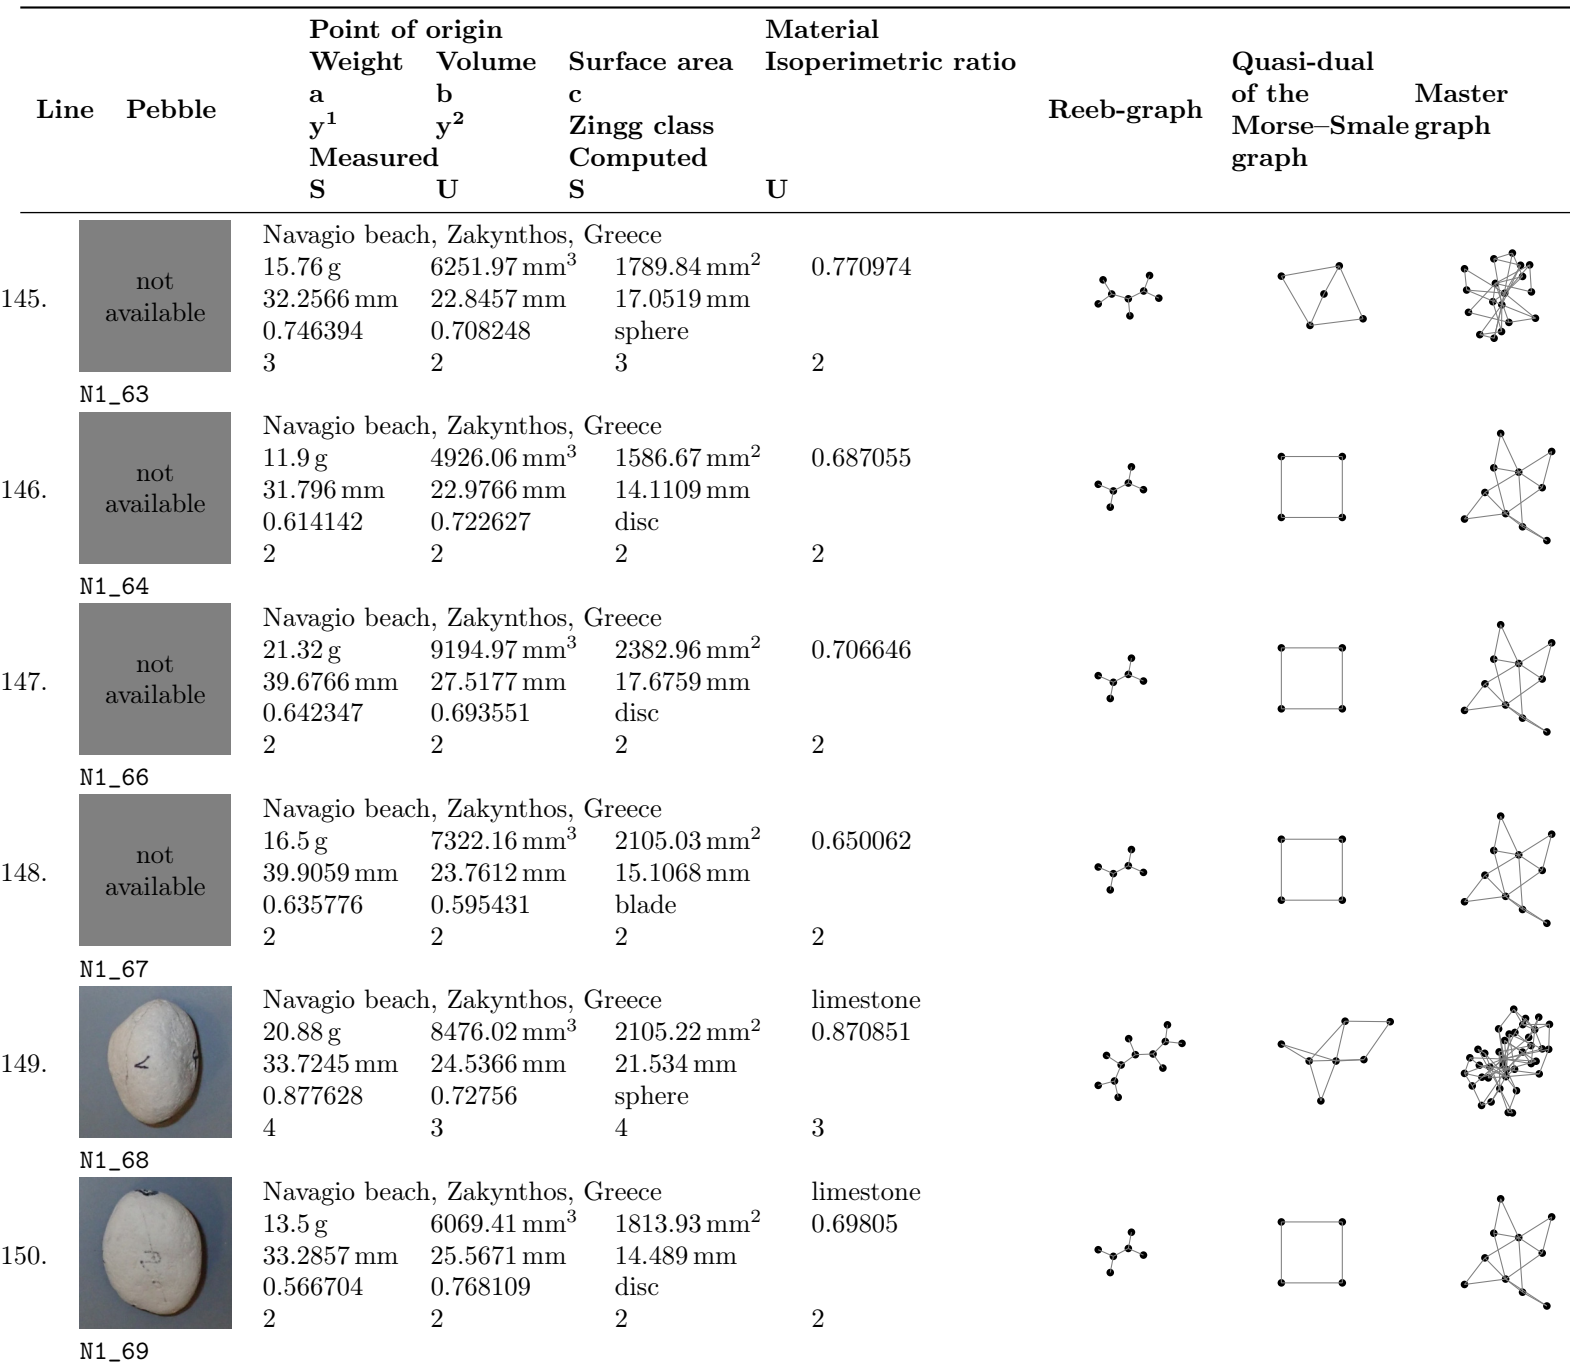  | 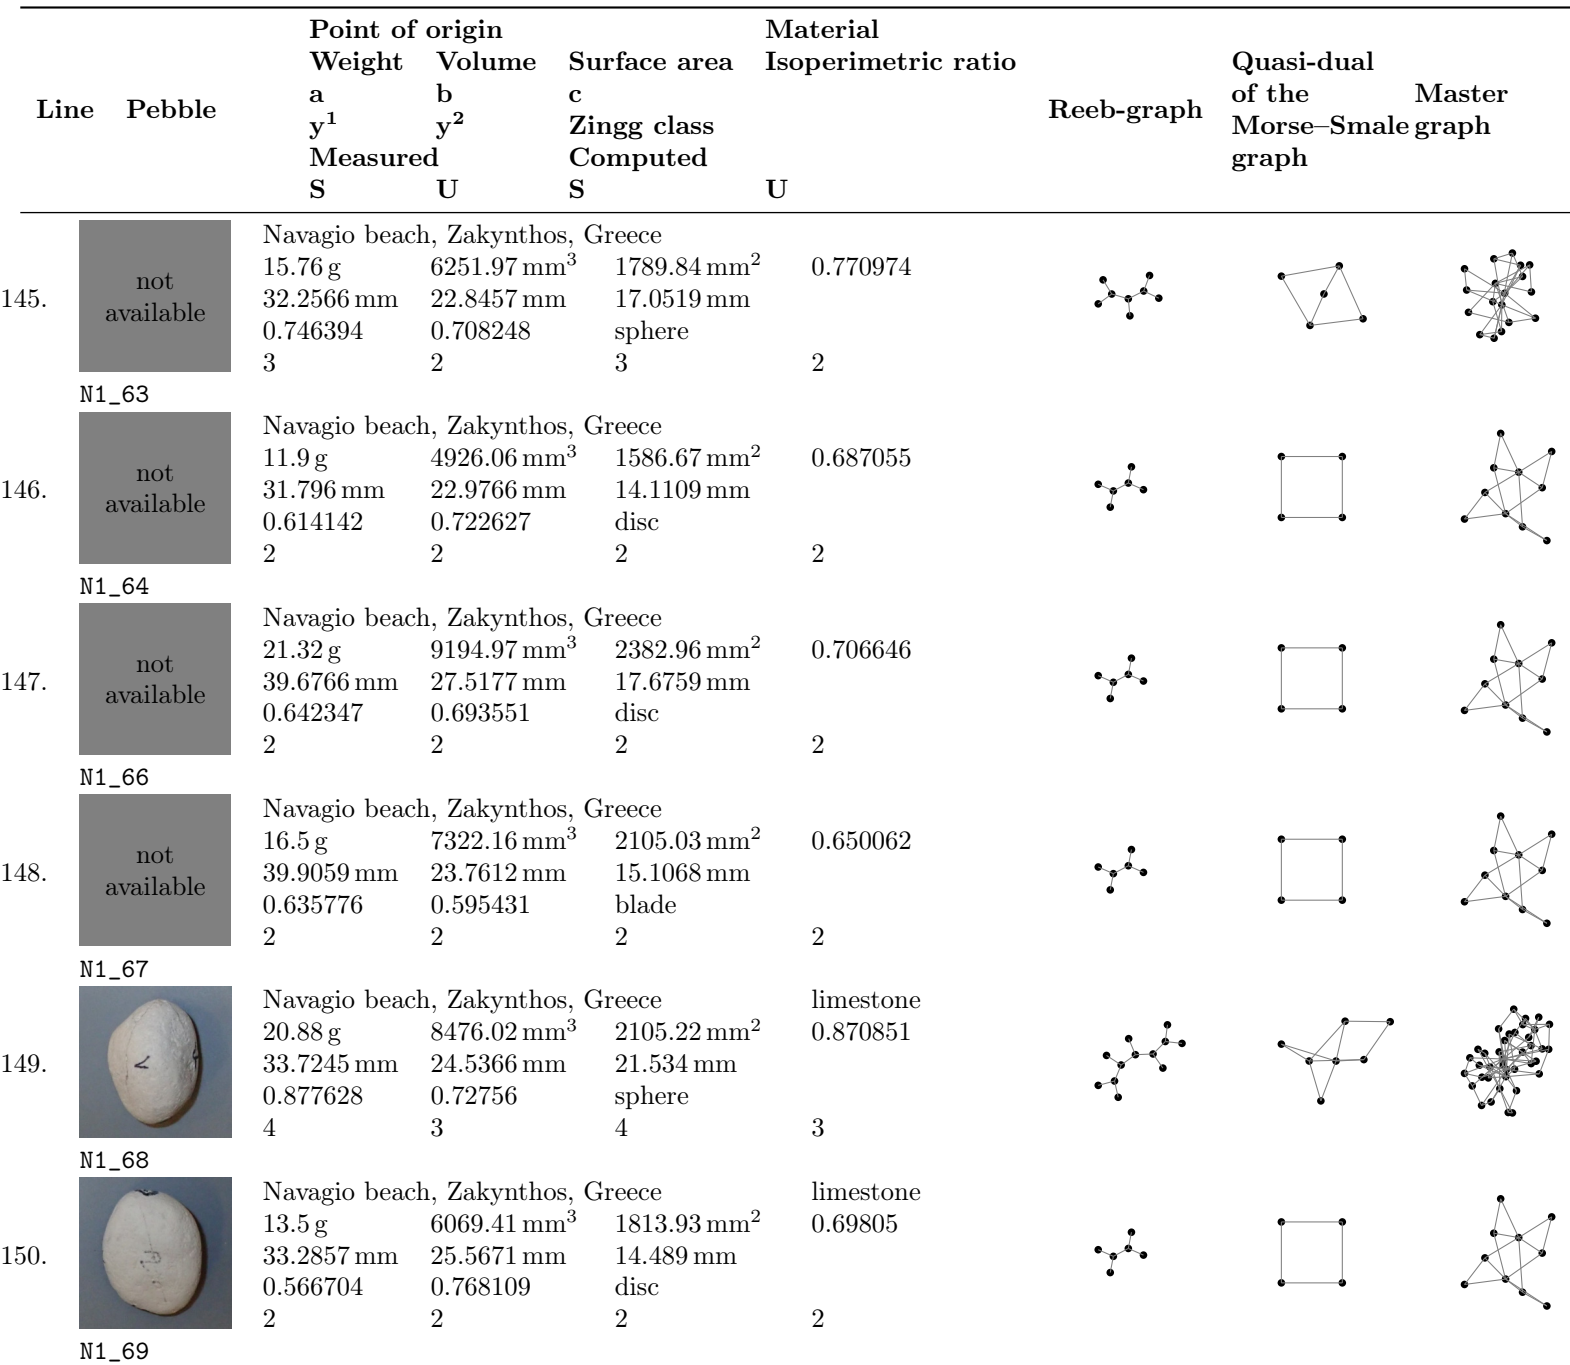  | 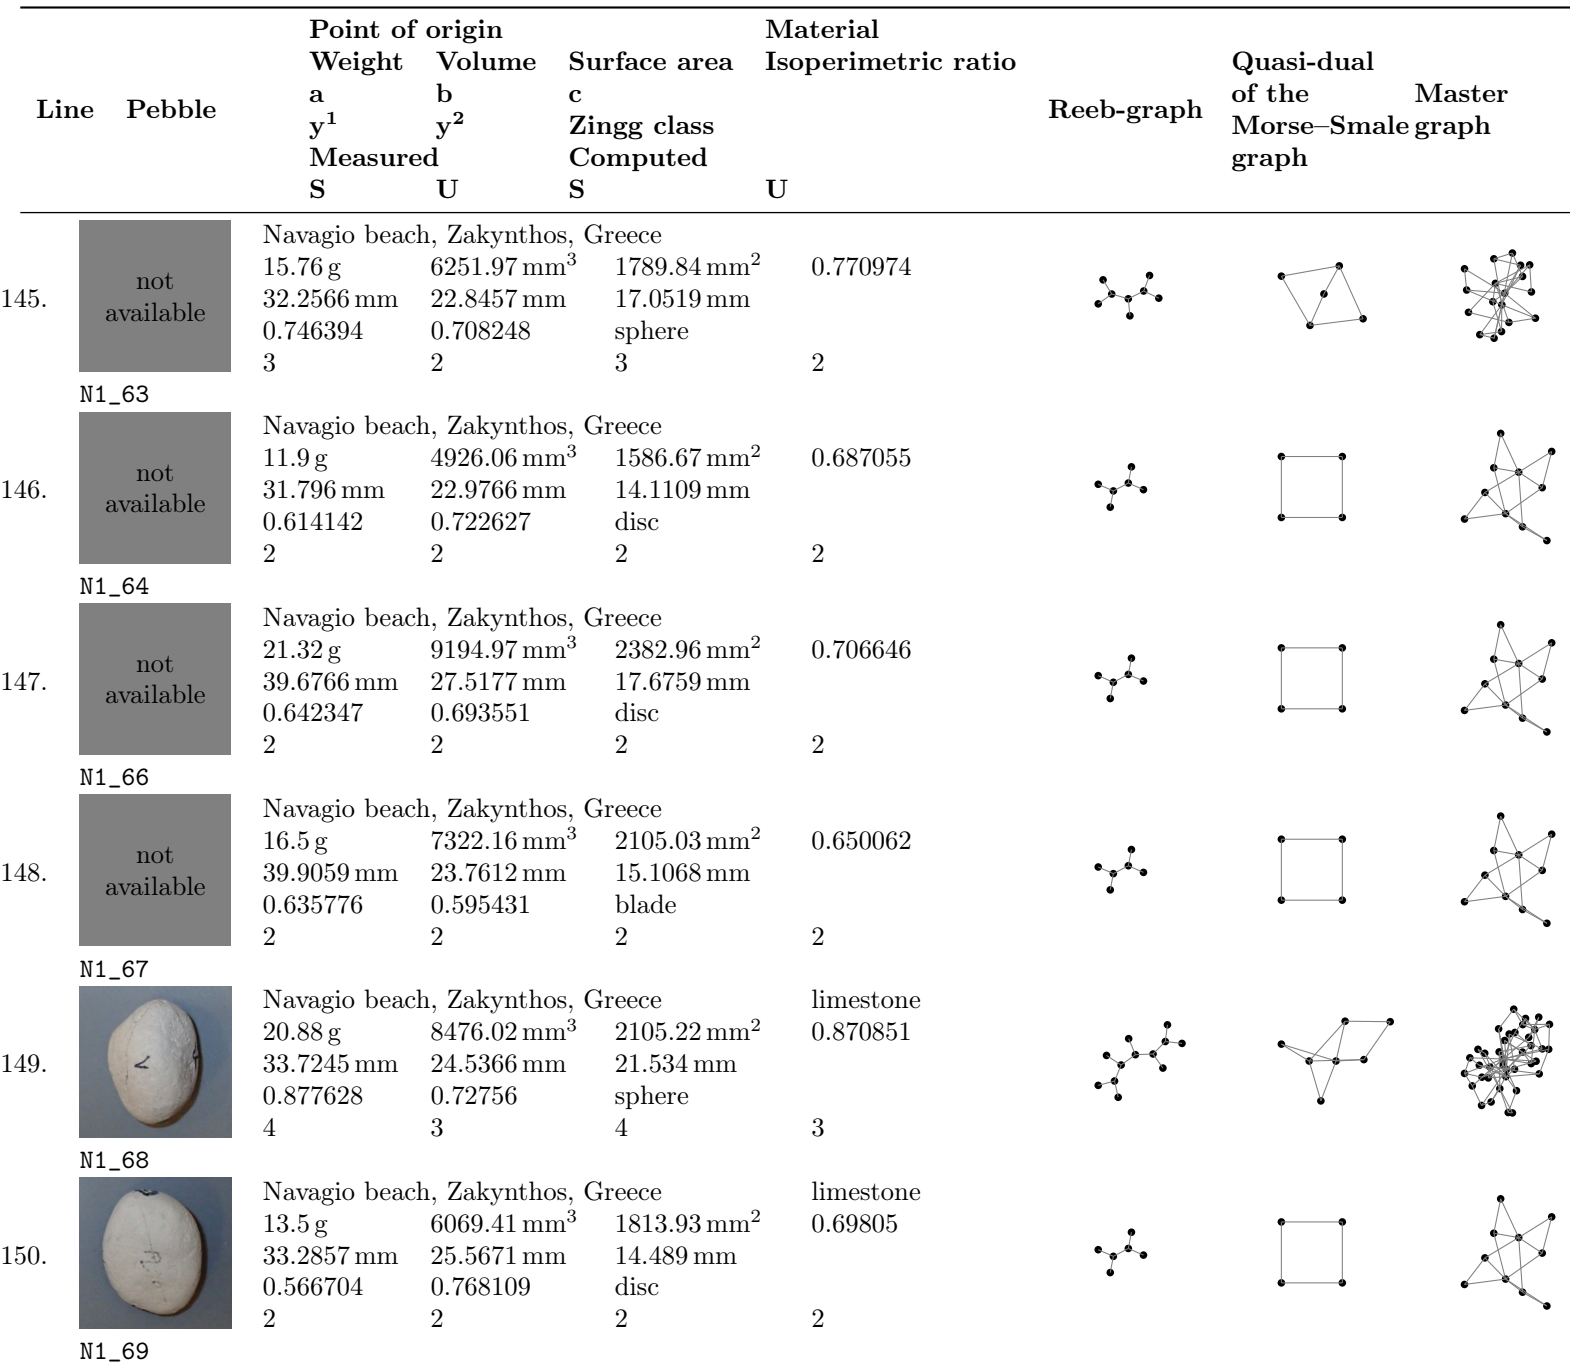  |
|       |                                                                                     | 16.5 g                               | 7322.16 mm <sup>3</sup>  | 2105.03 mm <sup>2</sup>                           |                                      |                                                                                       |                                                                                       |                                                                                       |
|       |                                                                                     | 39.9059 mm                           | 23.7612 mm               | 15.1068 mm                                        |                                      |                                                                                       |                                                                                       |                                                                                       |
|       |                                                                                     | 0.635776                             | 0.595431                 | blade                                             |                                      |                                                                                       |                                                                                       |                                                                                       |
|       |                                                                                     | 2                                    | 2                        | 2                                                 |                                      |                                                                                       |                                                                                       |                                                                                       |
| N1_67 |                                                                                     |                                      |                          |                                                   |                                      |                                                                                       |                                                                                       |                                                                                       |
| 149.  | 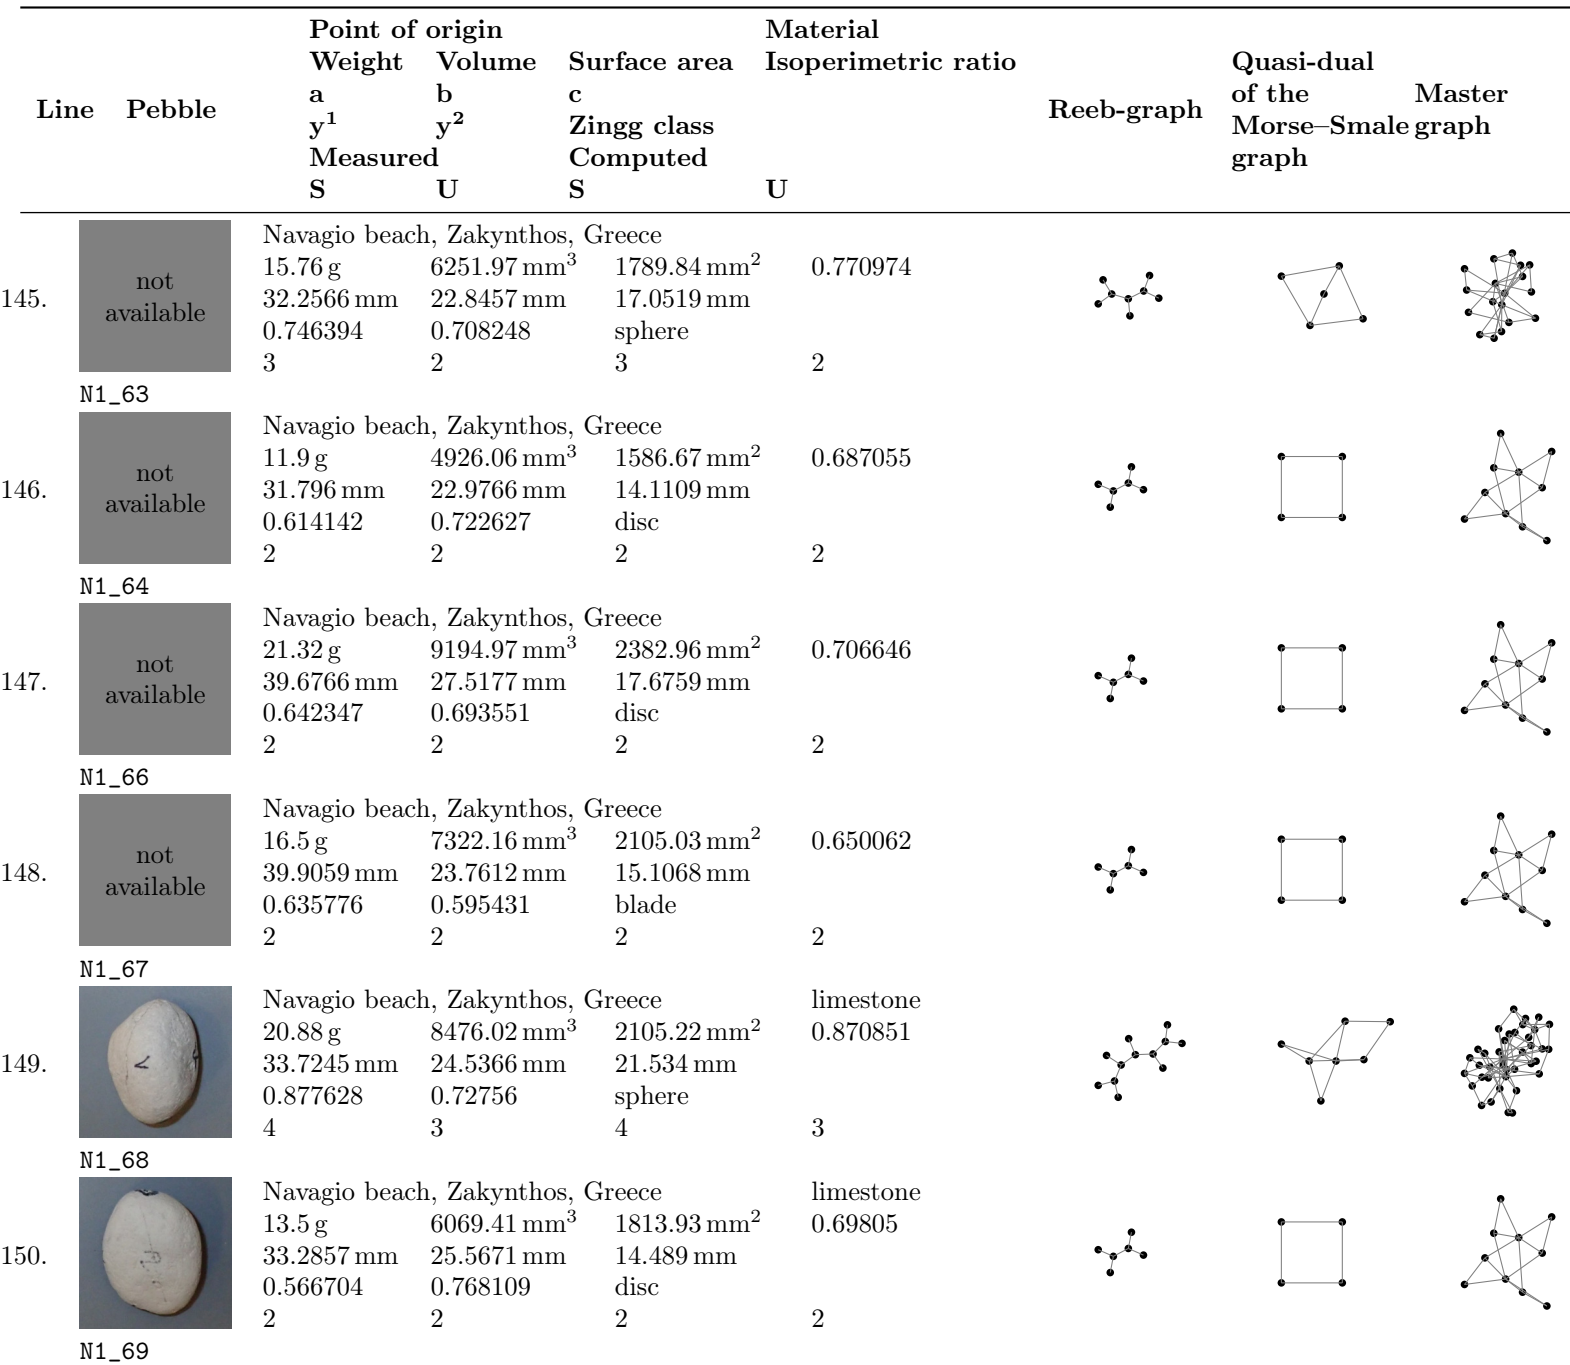 | Navagio beach, Zakynthos, Greece     |                          |                                                   | limestone<br>0.870851                | 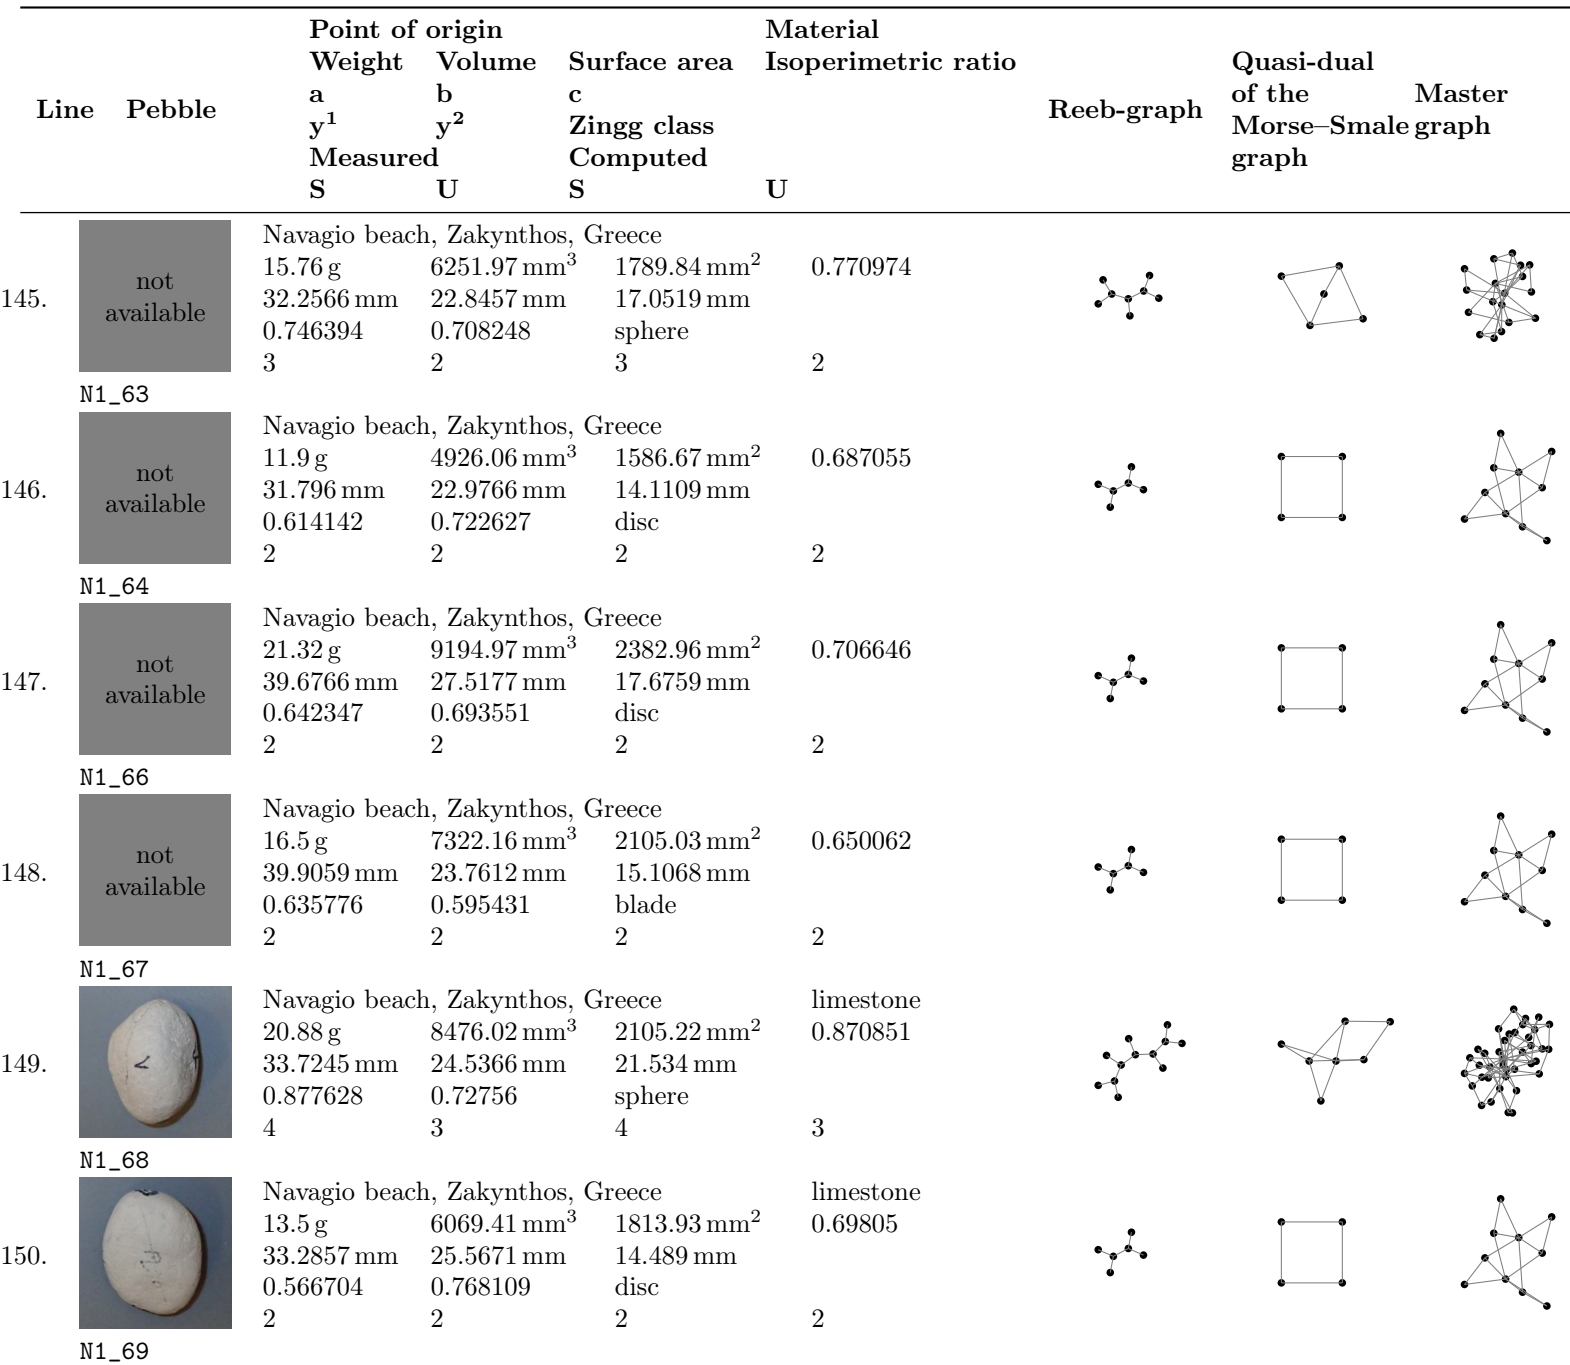 | 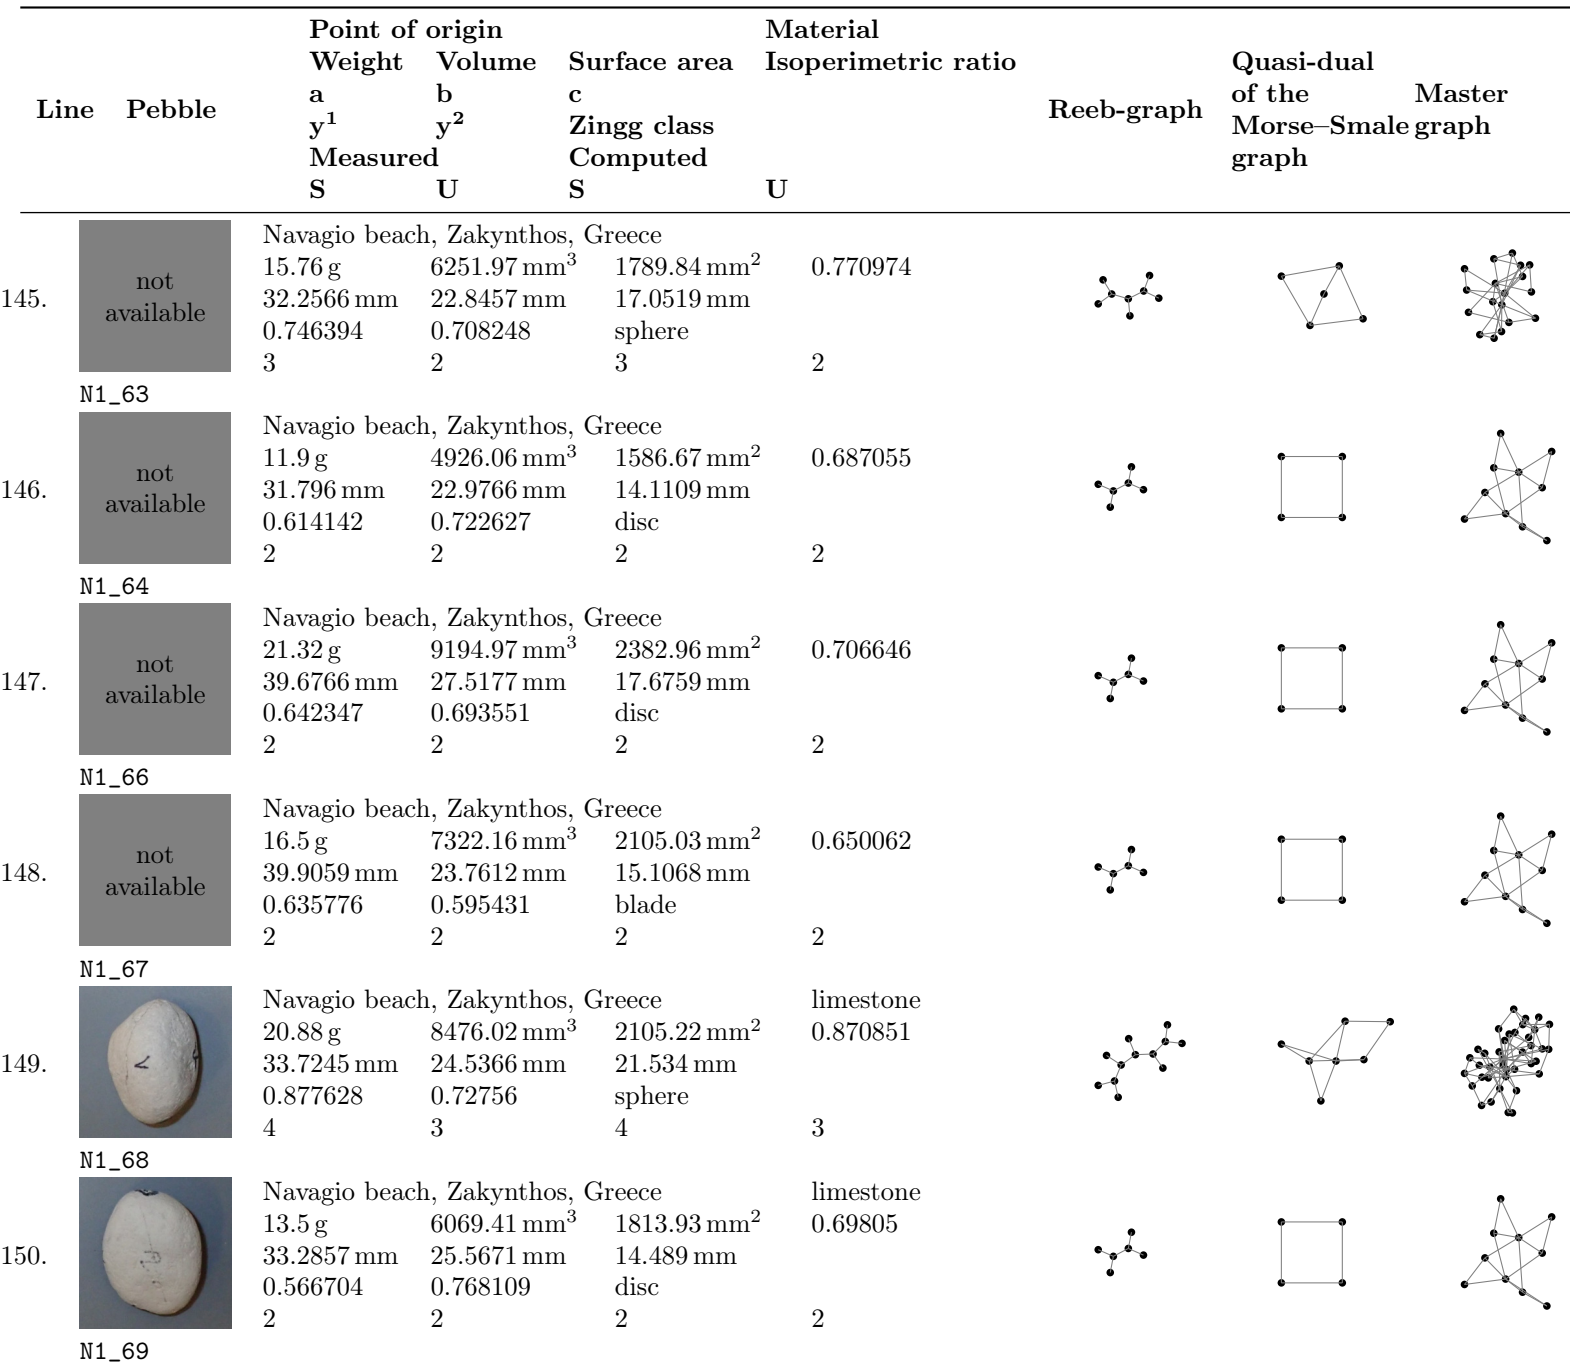 | 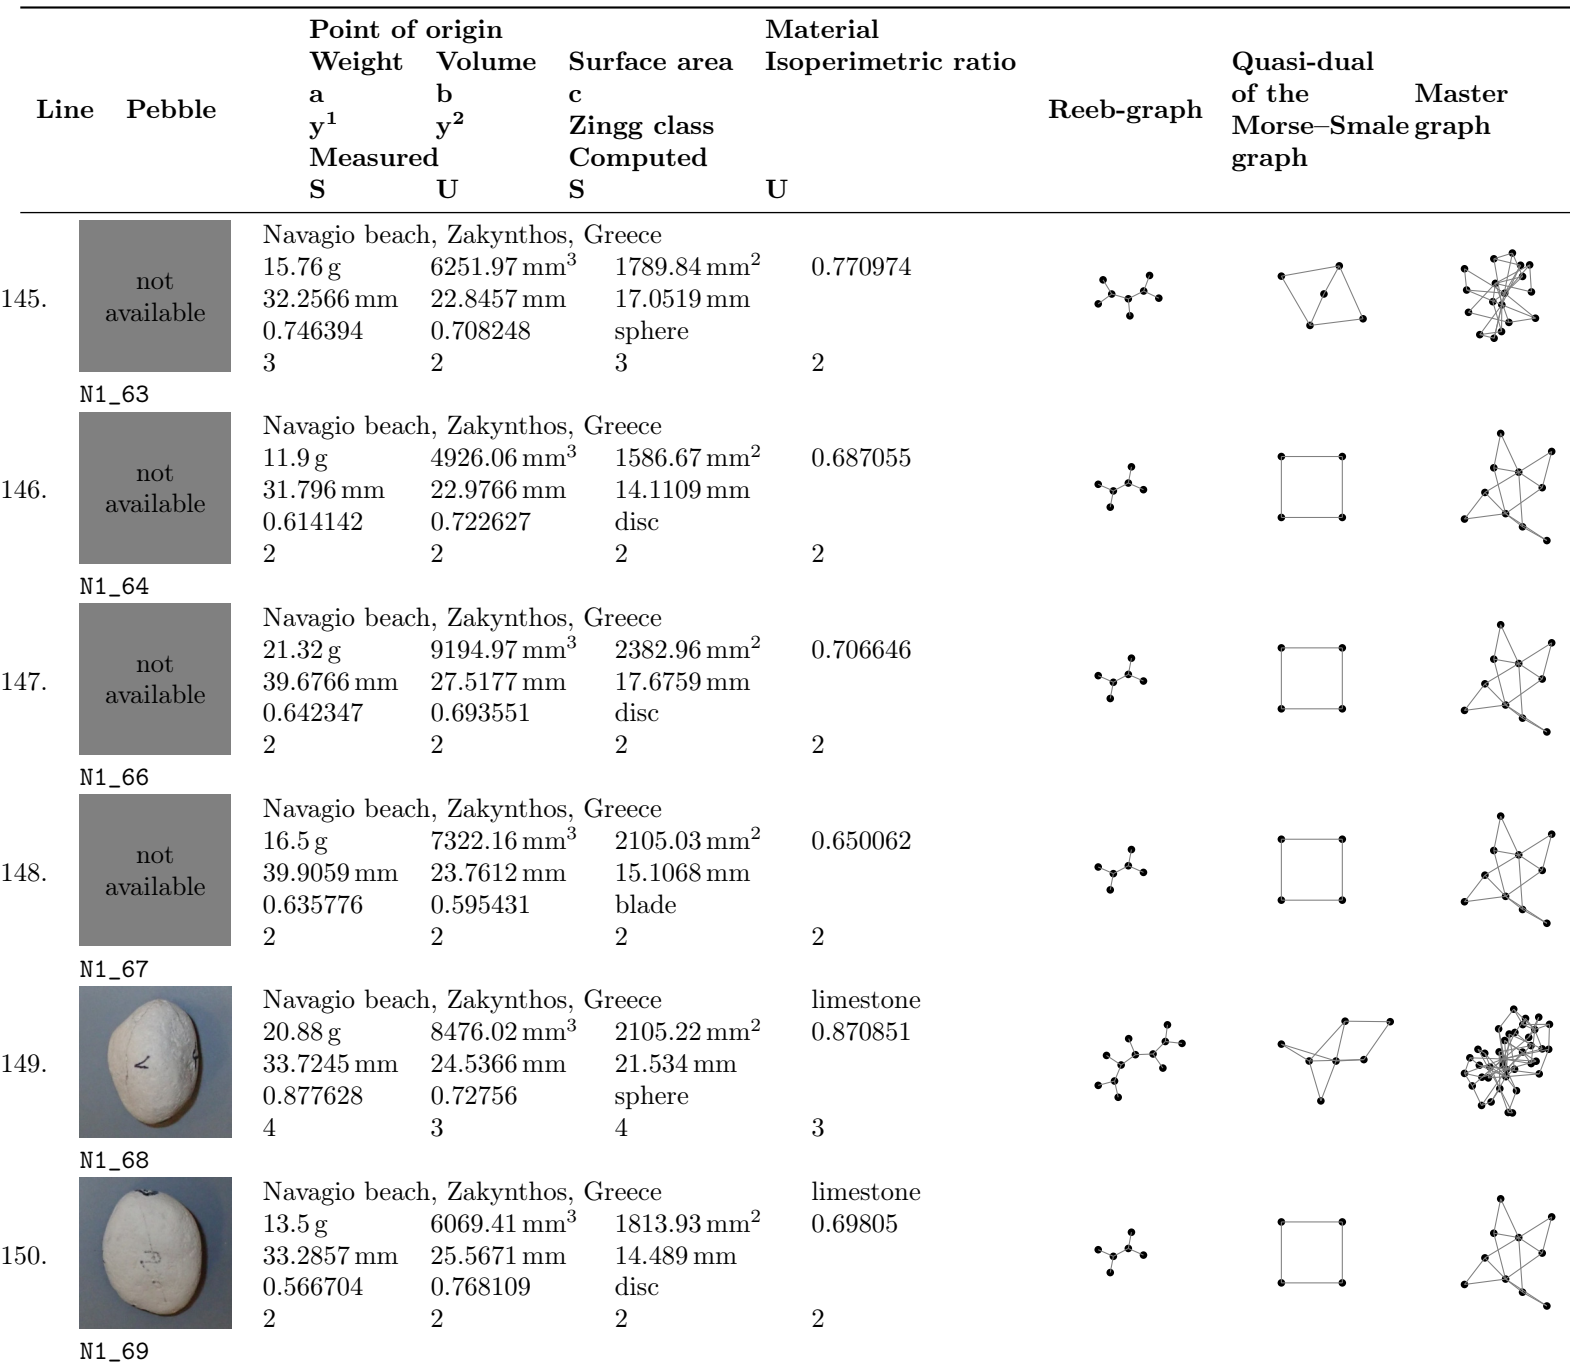 |
|       |                                                                                     | 20.88 g                              | 8476.02 mm <sup>3</sup>  | 2105.22 mm <sup>2</sup>                           |                                      |                                                                                       |                                                                                       |                                                                                       |
|       |                                                                                     | 33.7245 mm                           | 24.5366 mm               | 21.534 mm                                         |                                      |                                                                                       |                                                                                       |                                                                                       |
|       |                                                                                     | 0.877628                             | 0.72756                  | sphere                                            |                                      |                                                                                       |                                                                                       |                                                                                       |
|       |                                                                                     | 4                                    | 3                        | 4                                                 |                                      |                                                                                       |                                                                                       |                                                                                       |
| N1_68 |                                                                                     |                                      |                          |                                                   |                                      |                                                                                       |                                                                                       |                                                                                       |
| 150.  | 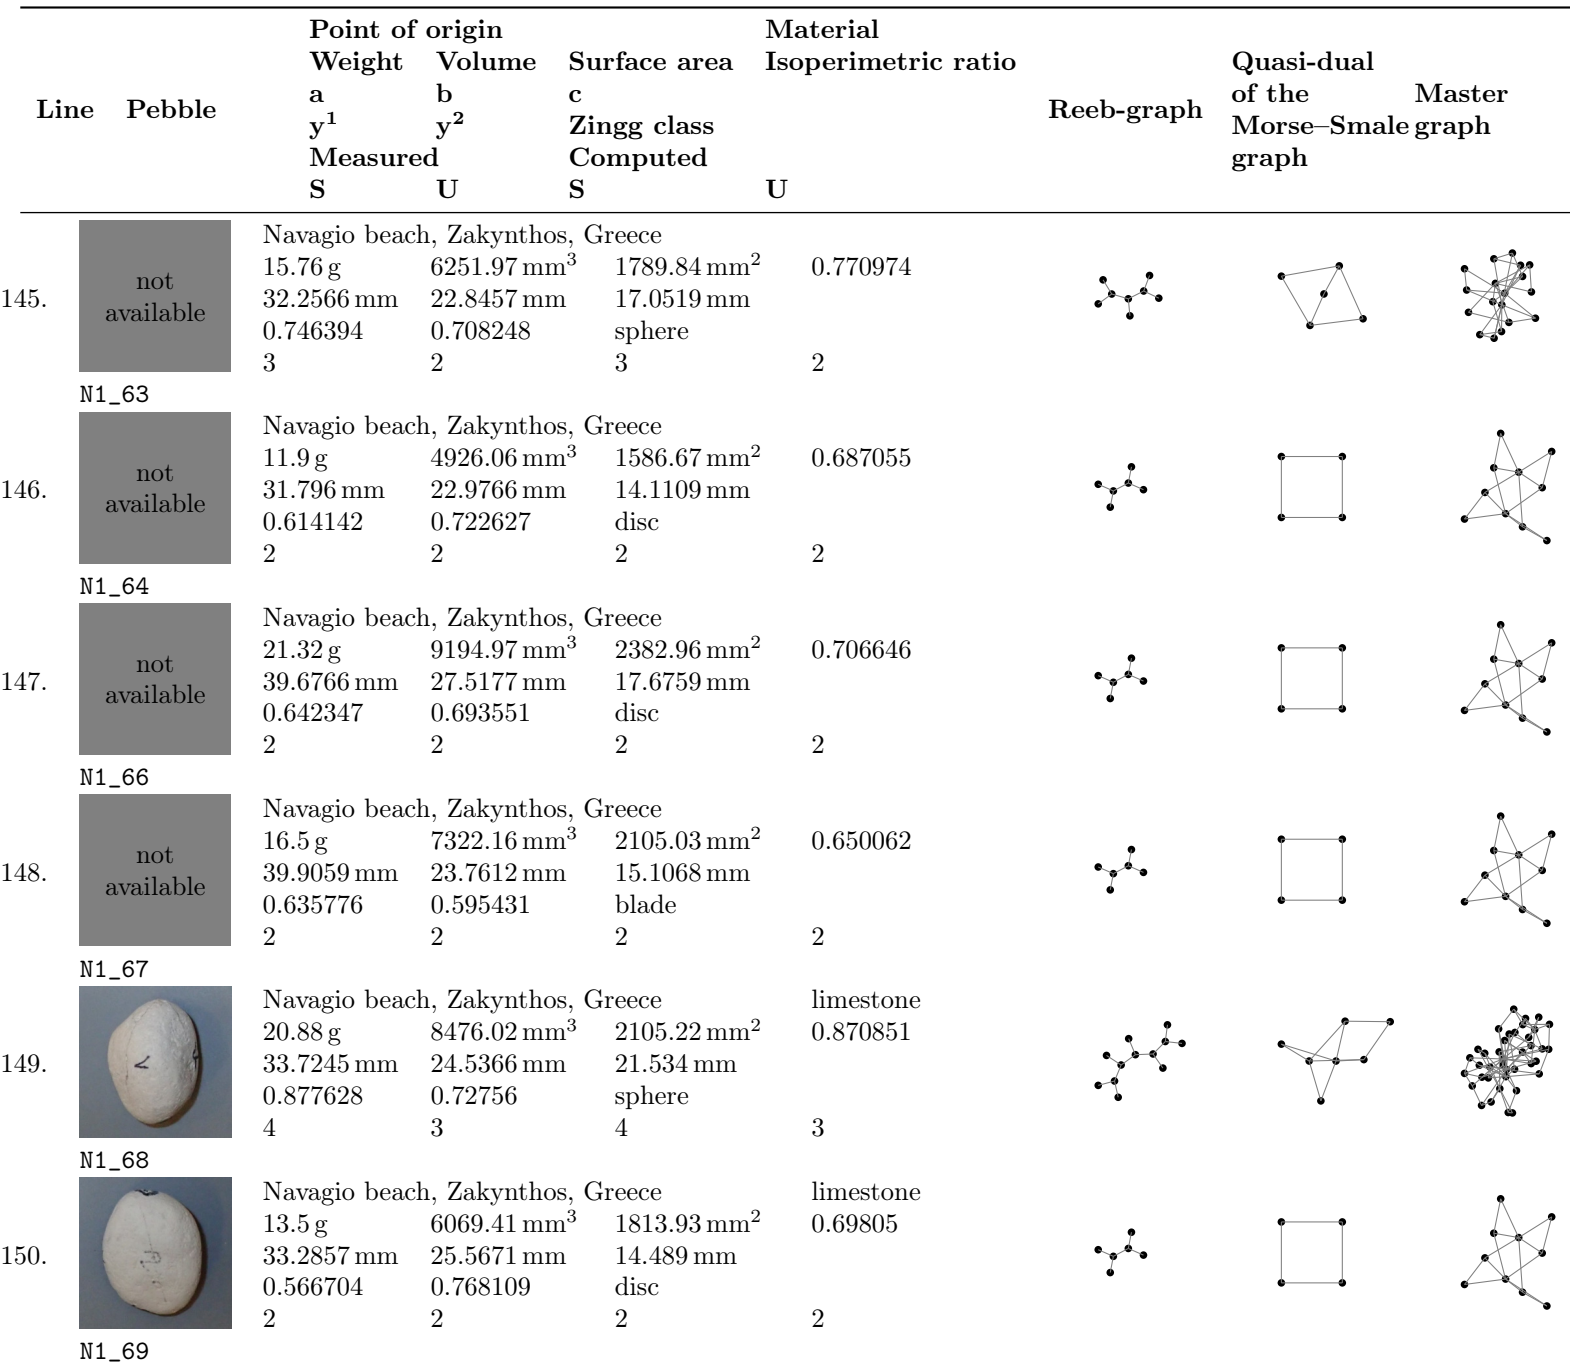 | Navagio beach, Zakynthos, Greece     |                          |                                                   | limestone<br>0.69805                 | 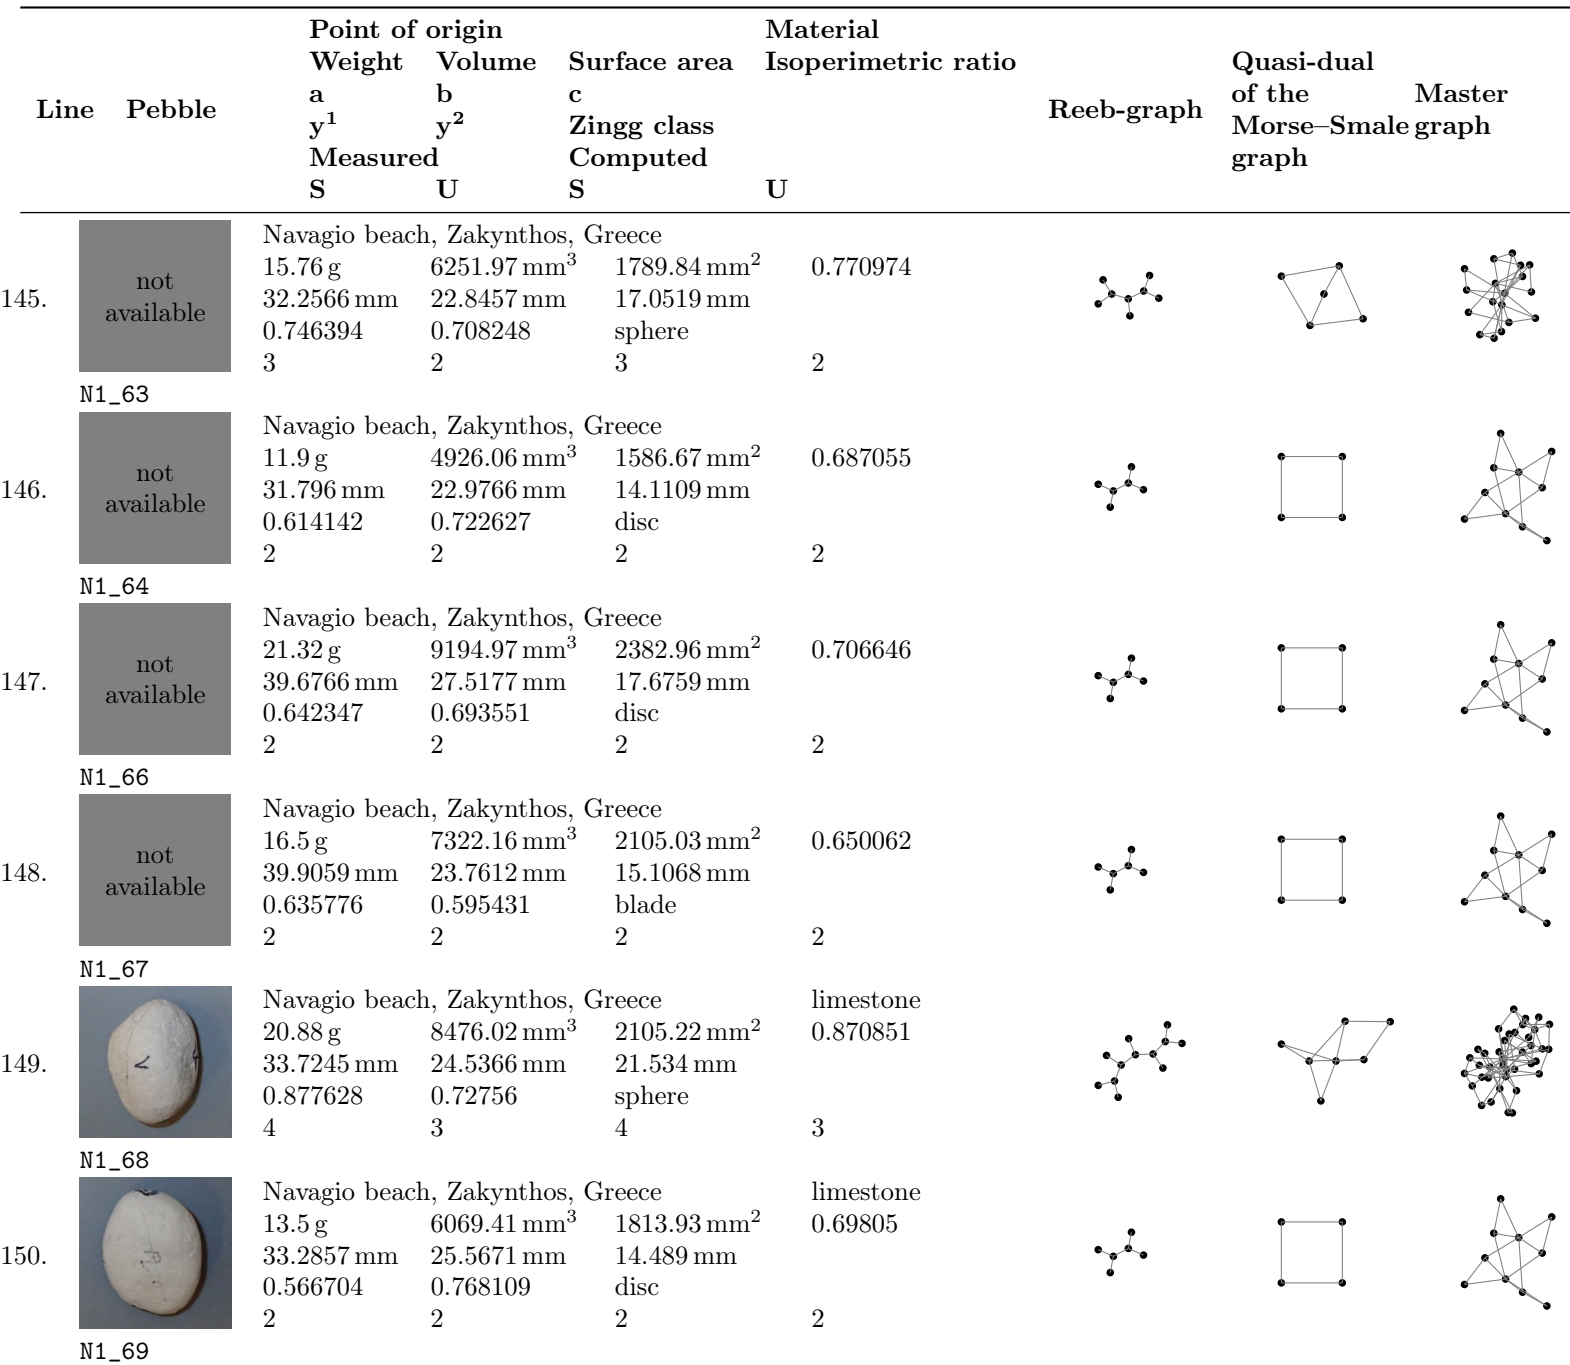 | 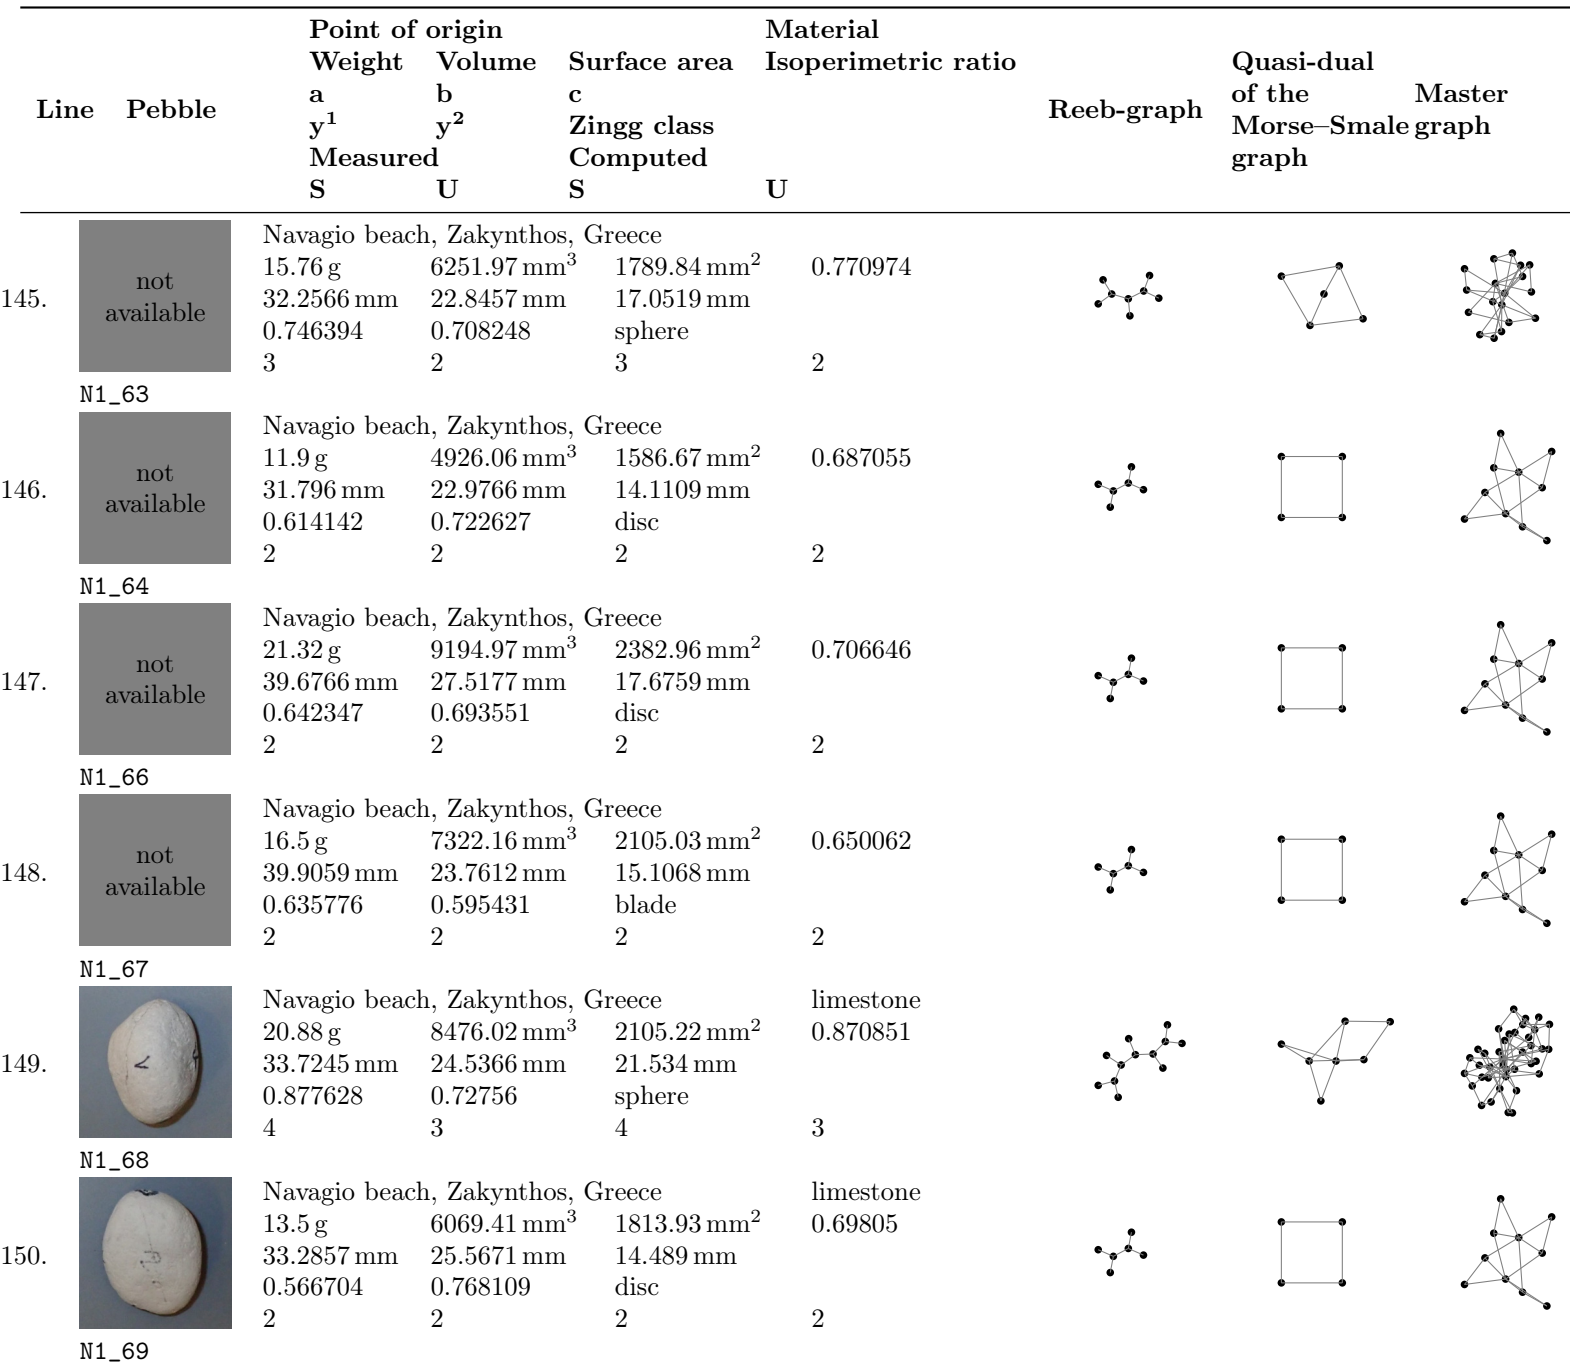 | 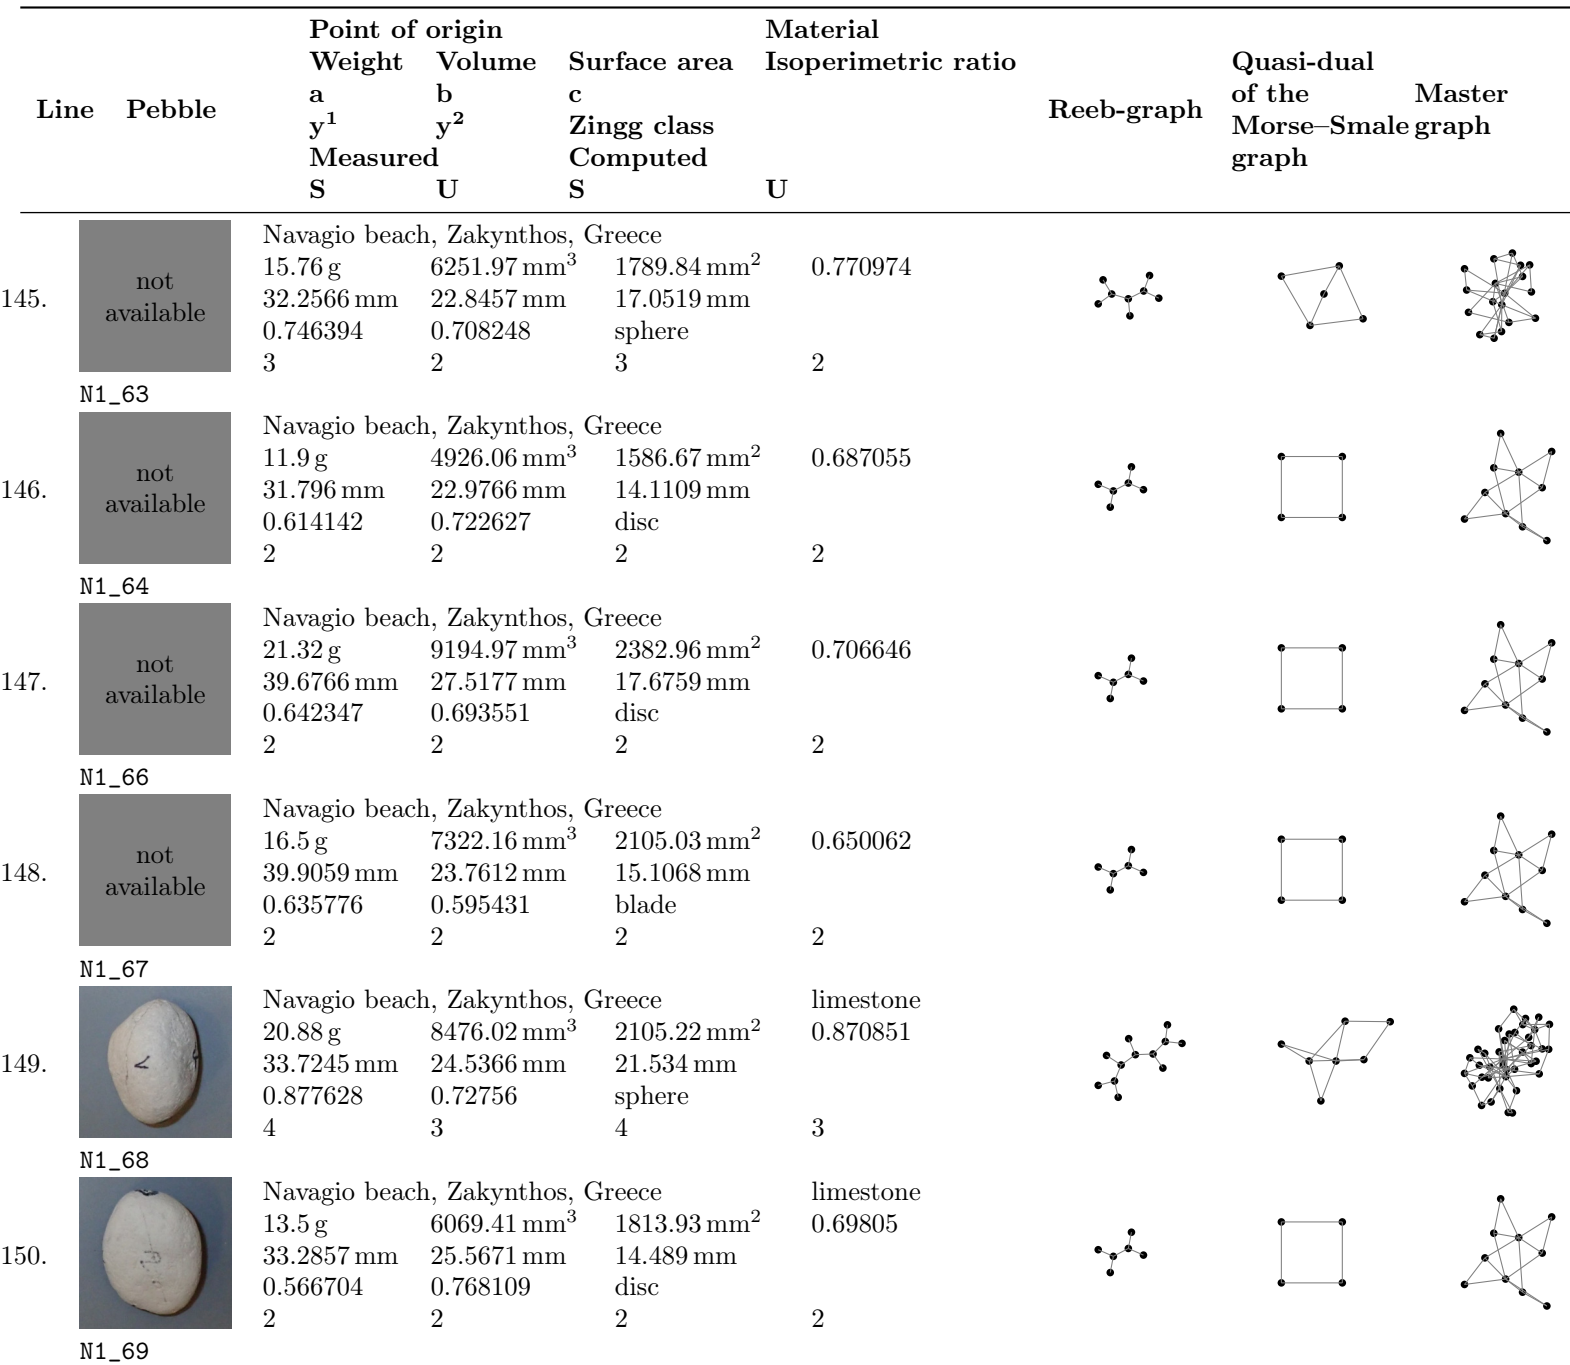 |
|       |                                                                                     | 13.5 g                               | 6069.41 mm <sup>3</sup>  | 1813.93 mm <sup>2</sup>                           |                                      |                                                                                       |                                                                                       |                                                                                       |
|       |                                                                                     | 33.2857 mm                           | 25.5671 mm               | 14.489 mm                                         |                                      |                                                                                       |                                                                                       |                                                                                       |
|       |                                                                                     | 0.566704                             | 0.768109                 | disc                                              |                                      |                                                                                       |                                                                                       |                                                                                       |
|       |                                                                                     | 2                                    | 2                        | 2                                                 |                                      |                                                                                       |                                                                                       |                                                                                       |
| N1_69 |                                                                                     |                                      |                          |                                                   |                                      |                                                                                       |                                                                                       |                                                                                       |

| Line | Pebble                                                                              | Point of origin                  |                         |                         | Material              | Reeb-graph                                                                            | Quasi-dual<br>of the<br>Morse–Smale<br>graph                                          | Master<br>graph                                                                       |
|------|-------------------------------------------------------------------------------------|----------------------------------|-------------------------|-------------------------|-----------------------|---------------------------------------------------------------------------------------|---------------------------------------------------------------------------------------|---------------------------------------------------------------------------------------|
|      |                                                                                     | Weight                           | Volume                  | Surface area            |                       |                                                                                       |                                                                                       |                                                                                       |
|      |                                                                                     | a                                | b                       | c                       |                       |                                                                                       |                                                                                       |                                                                                       |
|      |                                                                                     | y <sup>1</sup>                   | y <sup>2</sup>          | Zingg class             |                       |                                                                                       |                                                                                       |                                                                                       |
|      |                                                                                     | Measured                         | U                       | Computed                | U                     |                                                                                       |                                                                                       |                                                                                       |
| S    | S                                                                                   | S                                | S                       | S                       | S                     |                                                                                       |                                                                                       |                                                                                       |
| 151. | 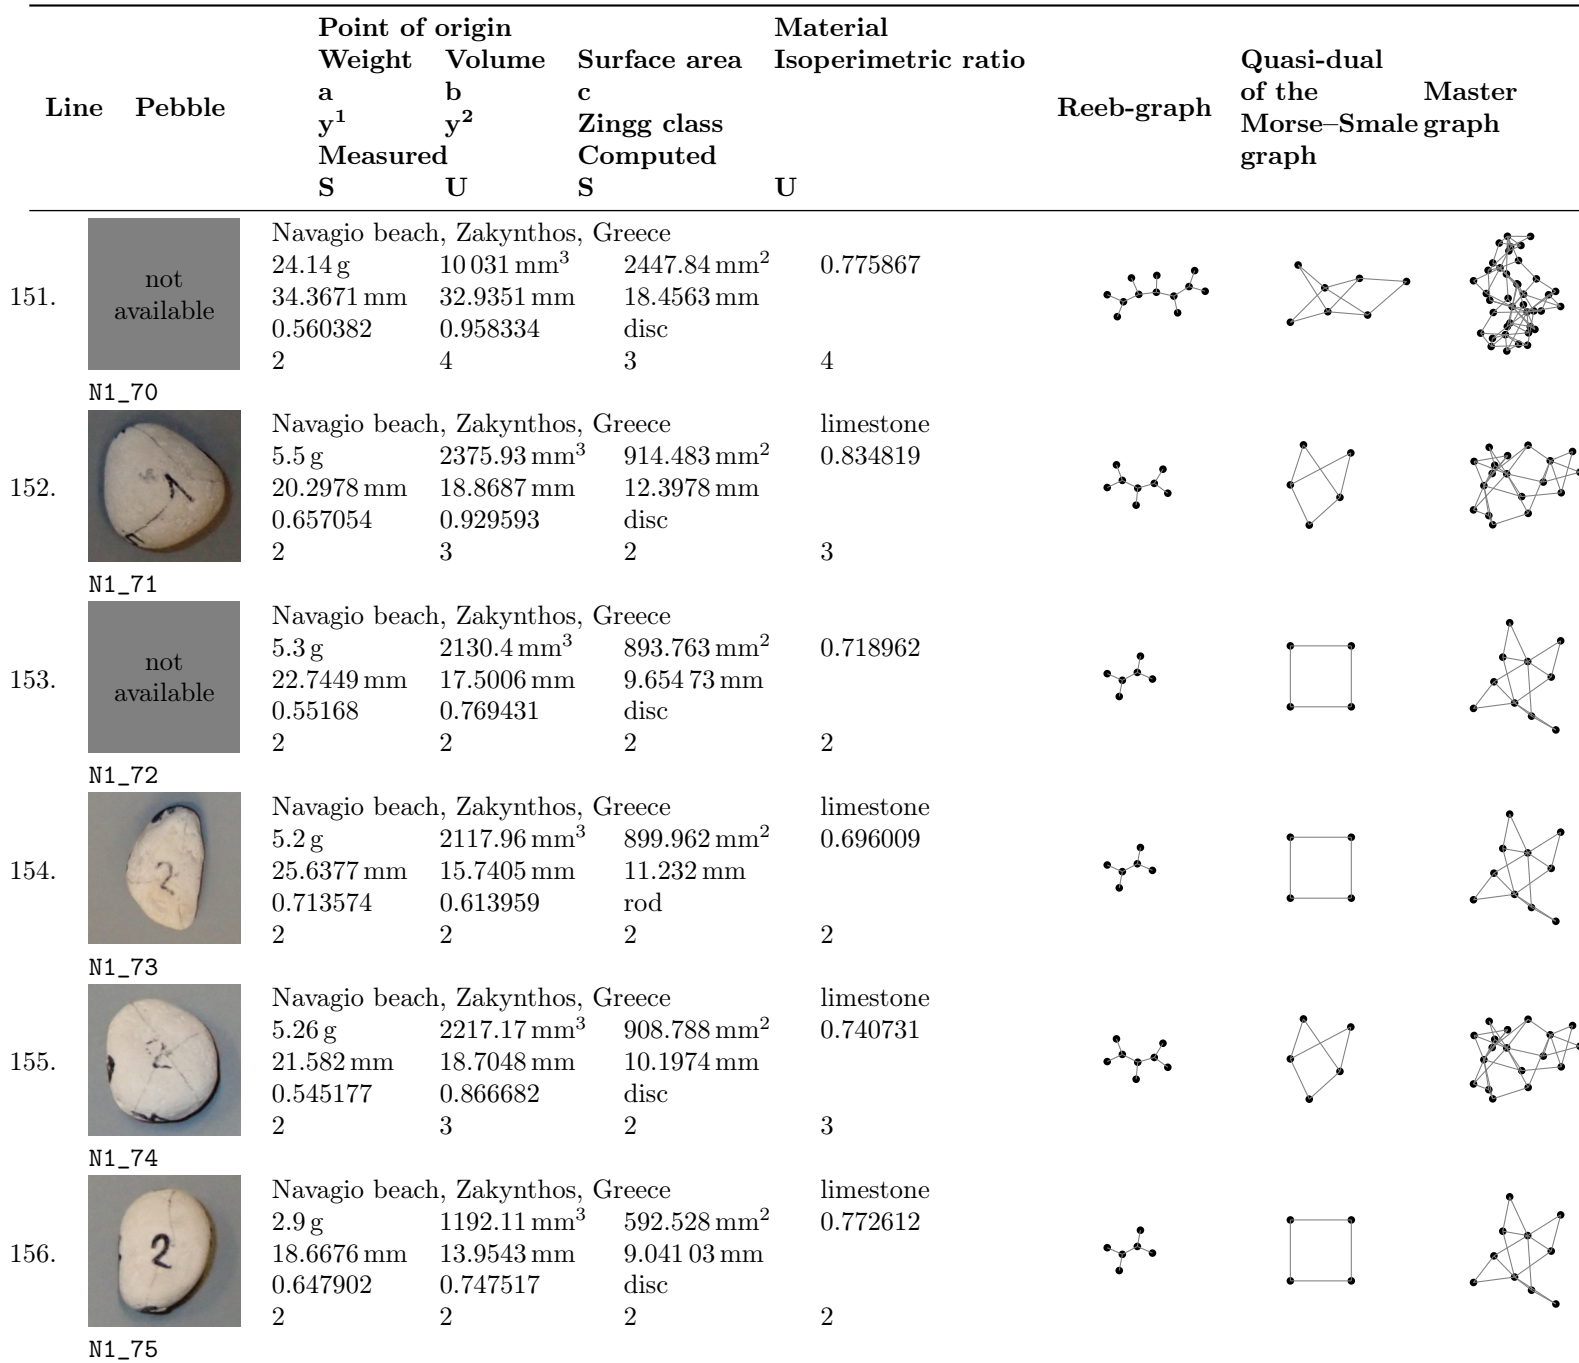   | Navagio beach, Zakynthos, Greece |                         |                         | 0.775867              | 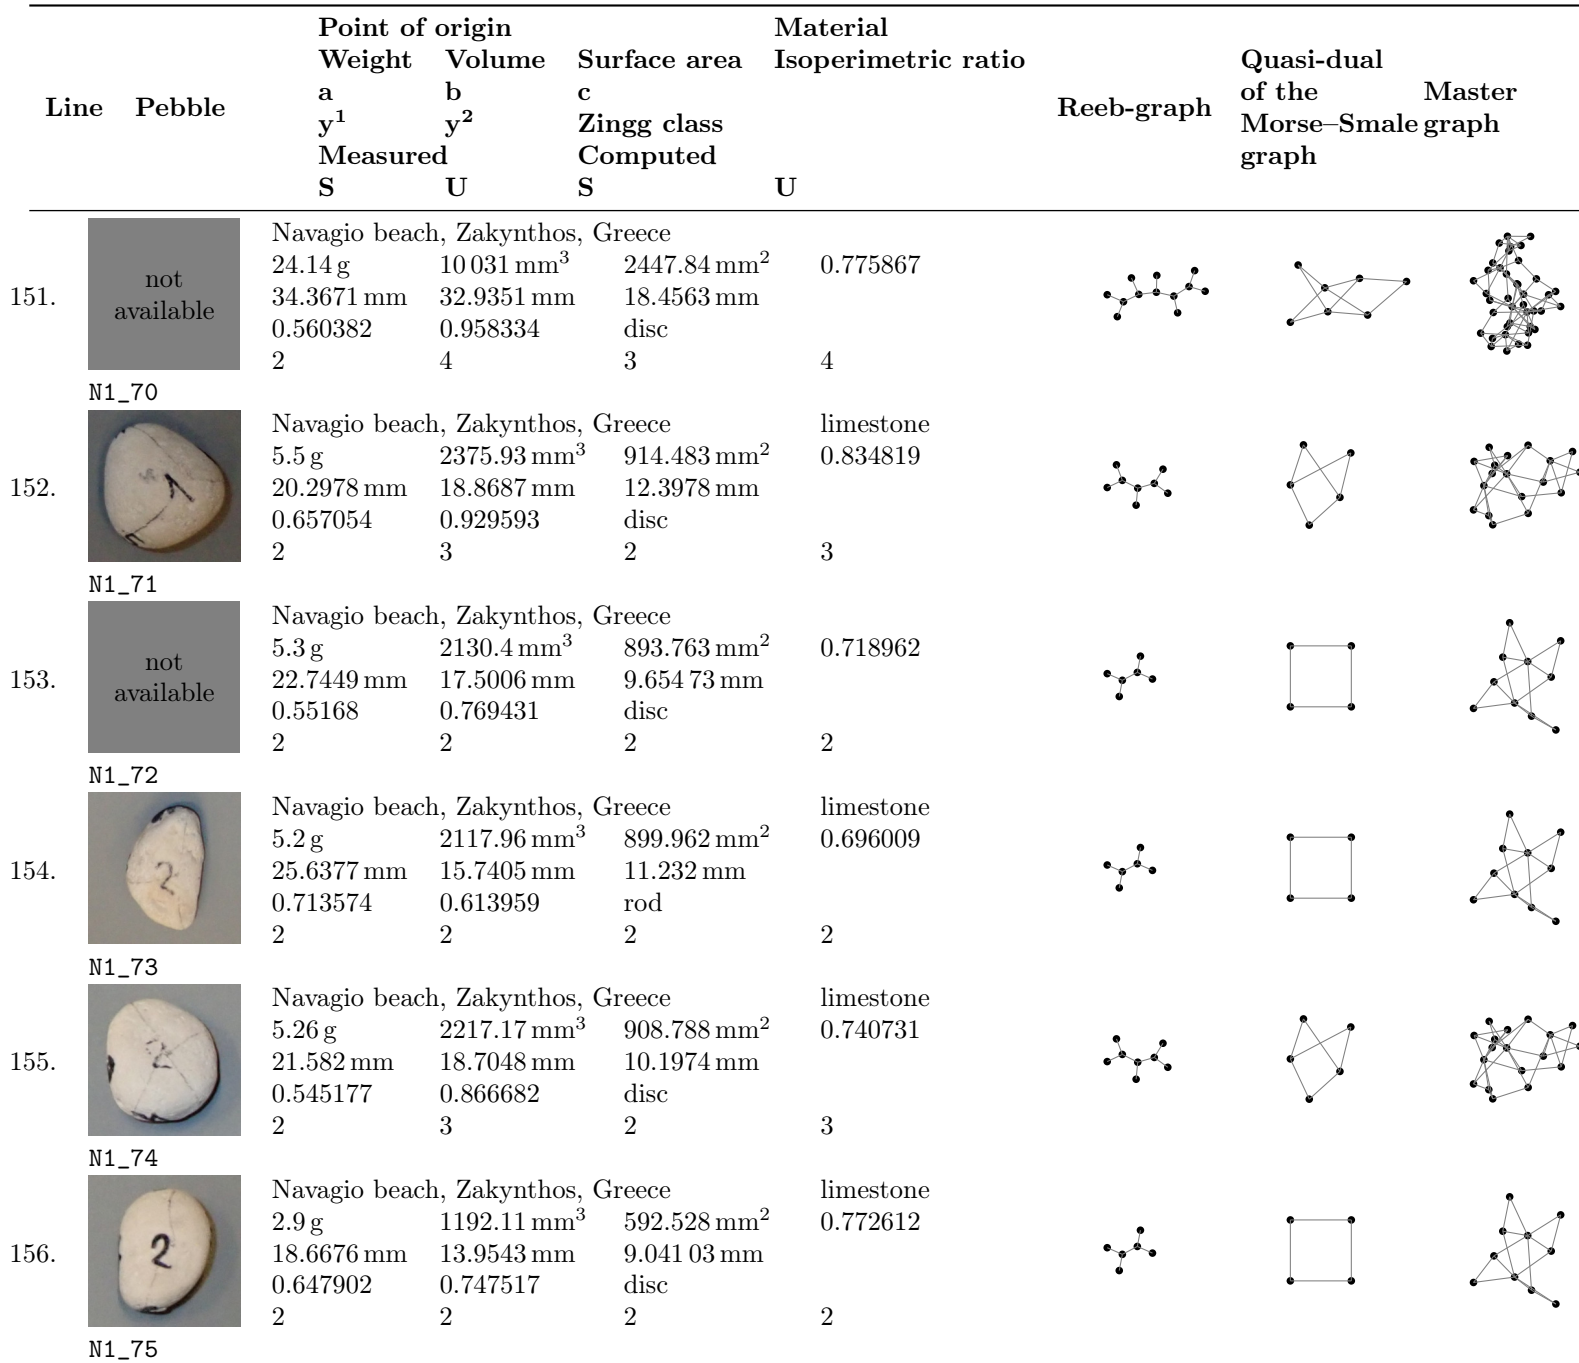   | 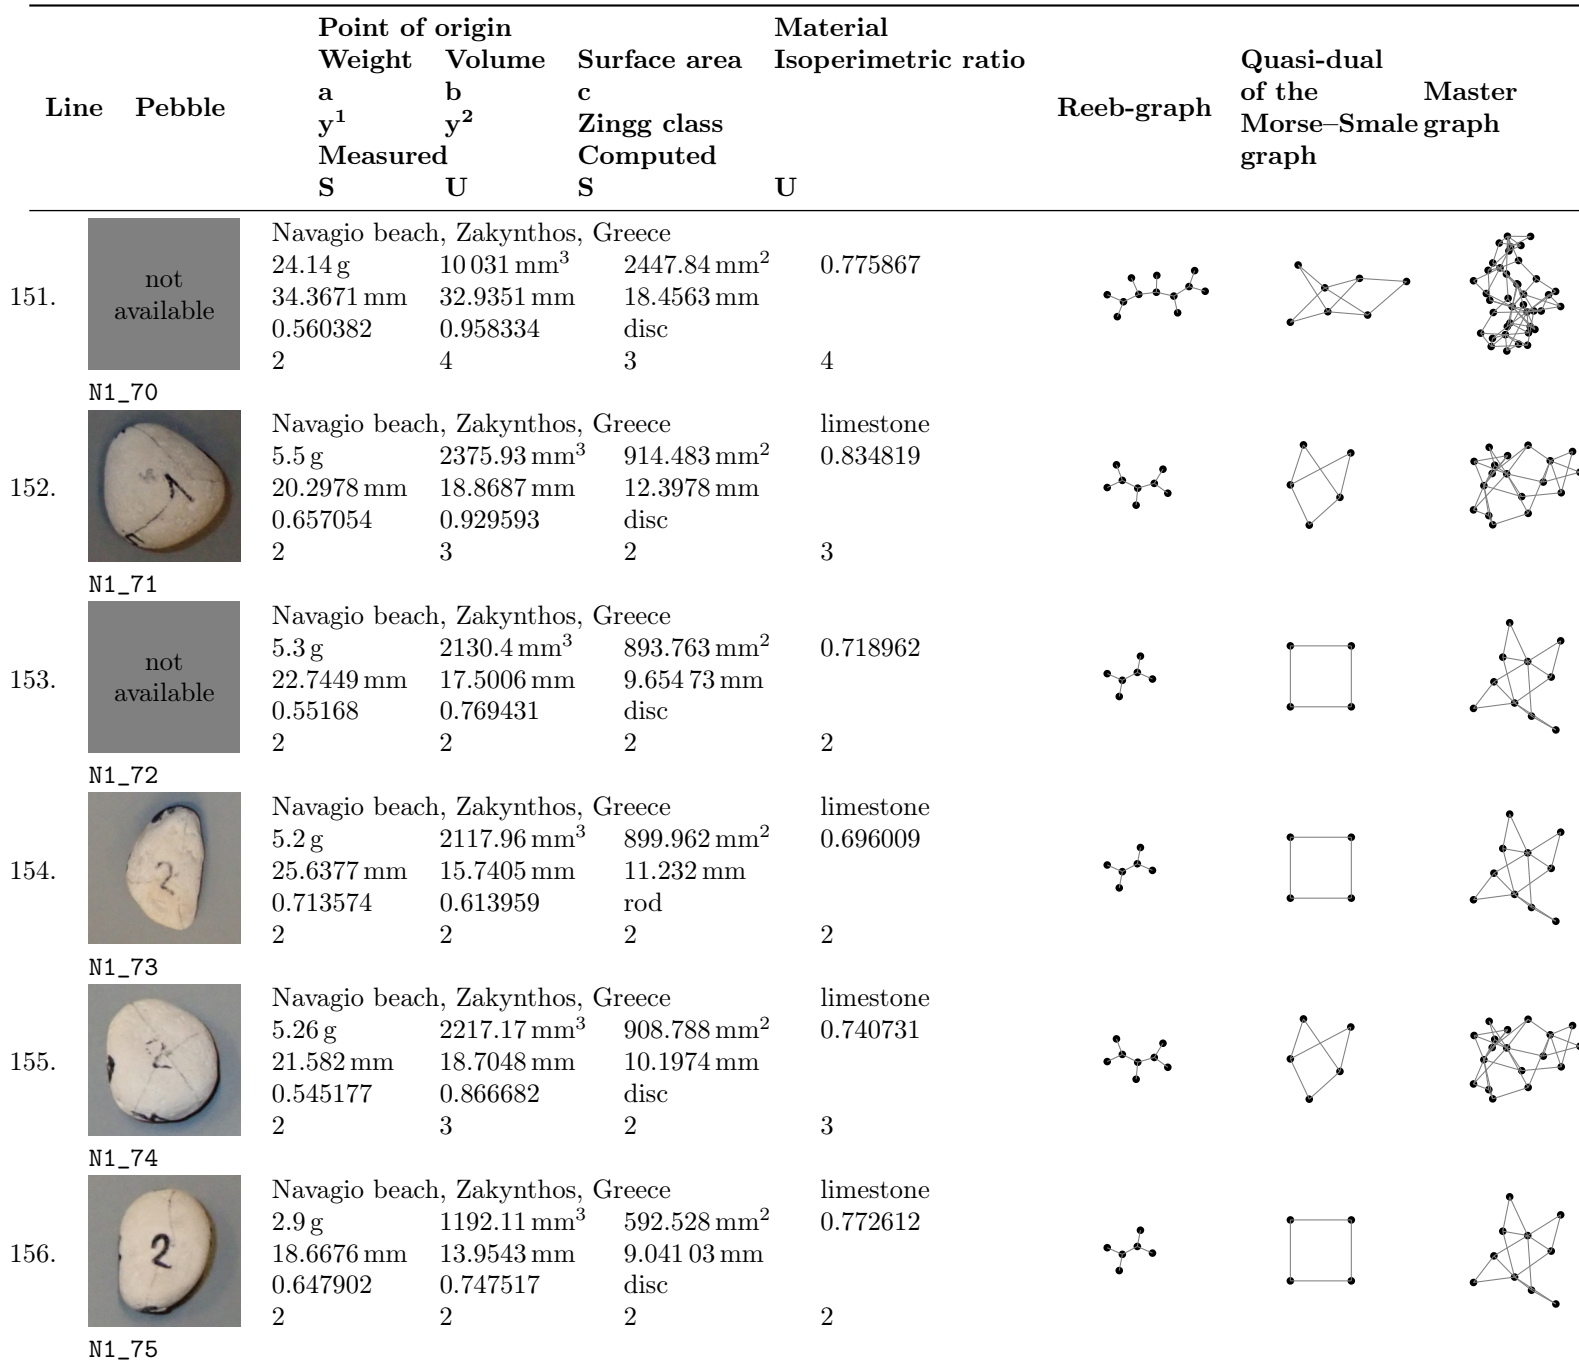   | 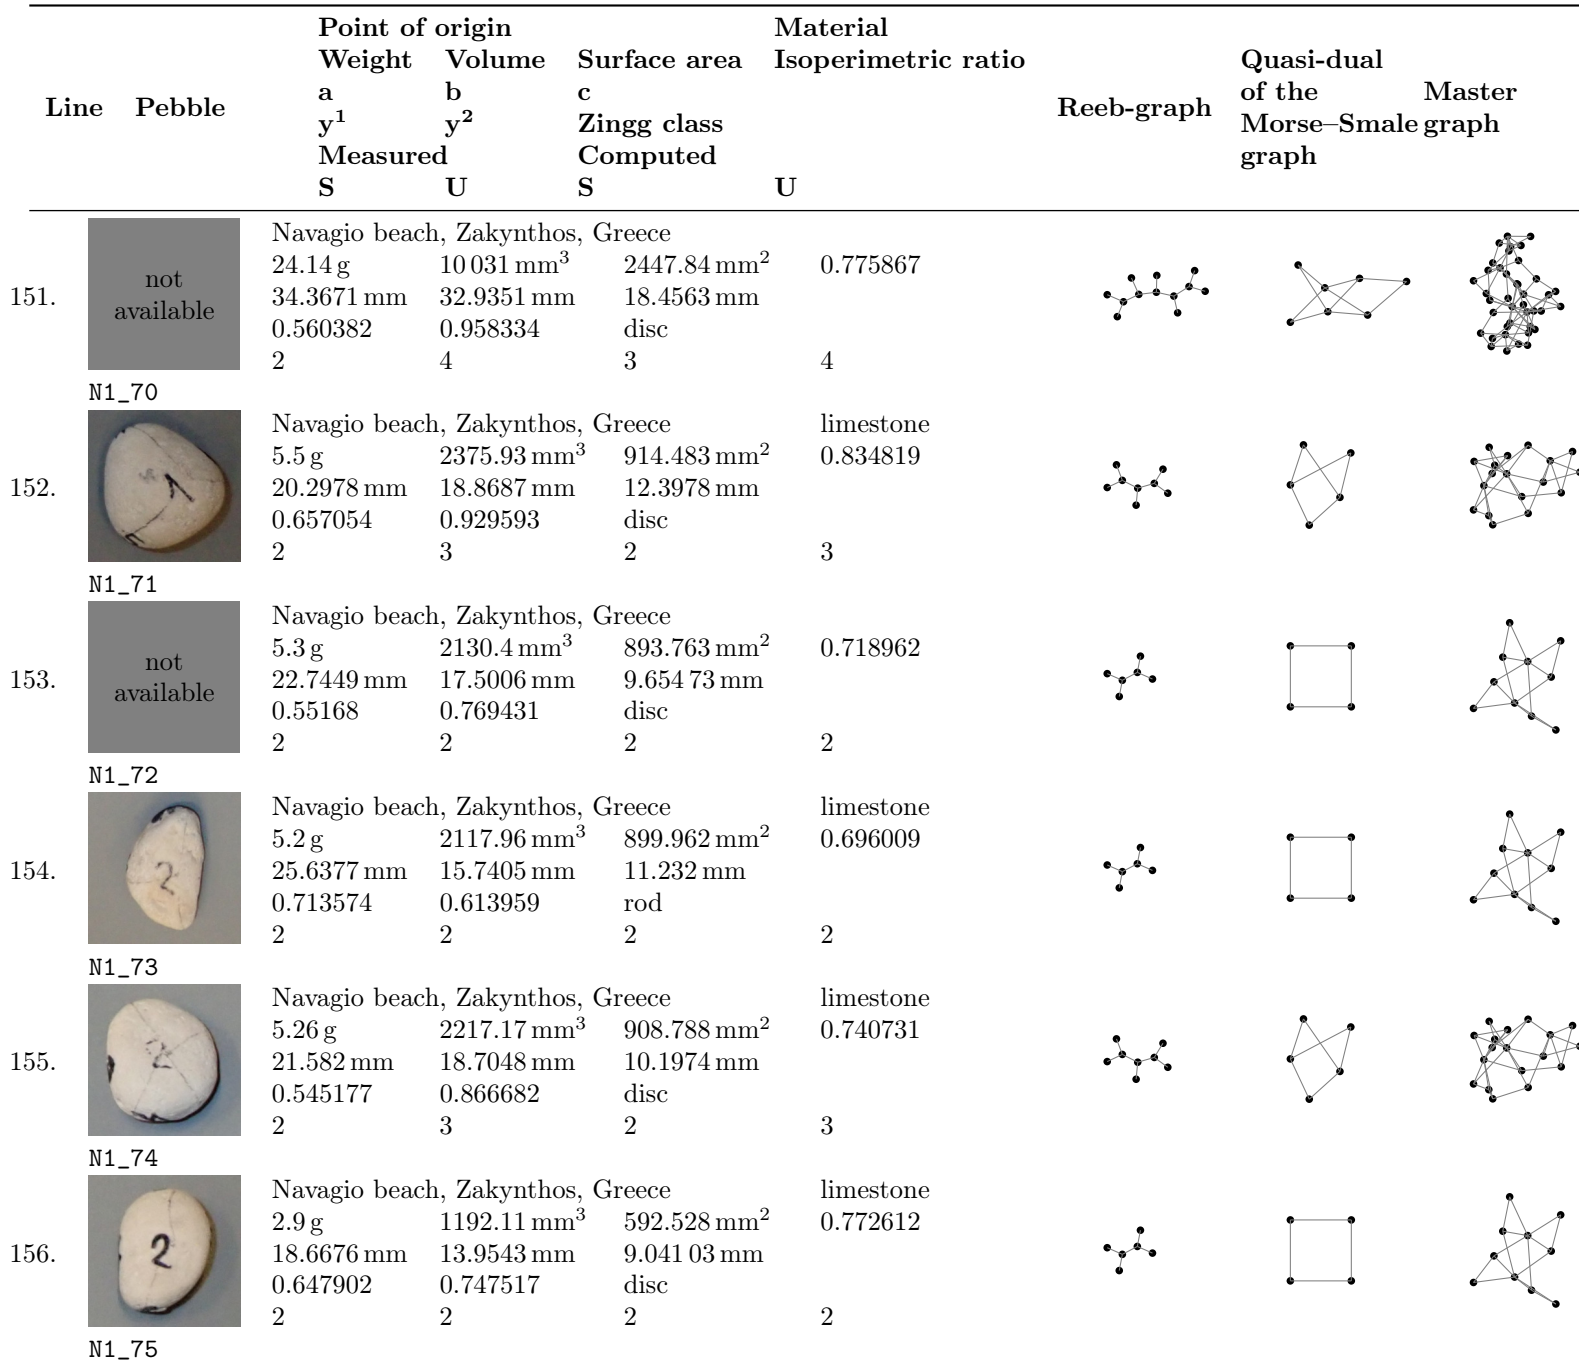   |
|      |                                                                                     | 24.14 g                          | 10 031 mm <sup>3</sup>  | 2447.84 mm <sup>2</sup> |                       |                                                                                       |                                                                                       |                                                                                       |
|      |                                                                                     | 34.3671 mm                       | 32.9351 mm              | 18.4563 mm              |                       |                                                                                       |                                                                                       |                                                                                       |
|      |                                                                                     | 0.560382                         | 0.958334                | disc                    |                       |                                                                                       |                                                                                       |                                                                                       |
|      |                                                                                     | 2                                | 4                       | 3                       |                       |                                                                                       |                                                                                       |                                                                                       |
|      | N1_70                                                                               |                                  |                         |                         |                       |                                                                                       |                                                                                       |                                                                                       |
| 152. | 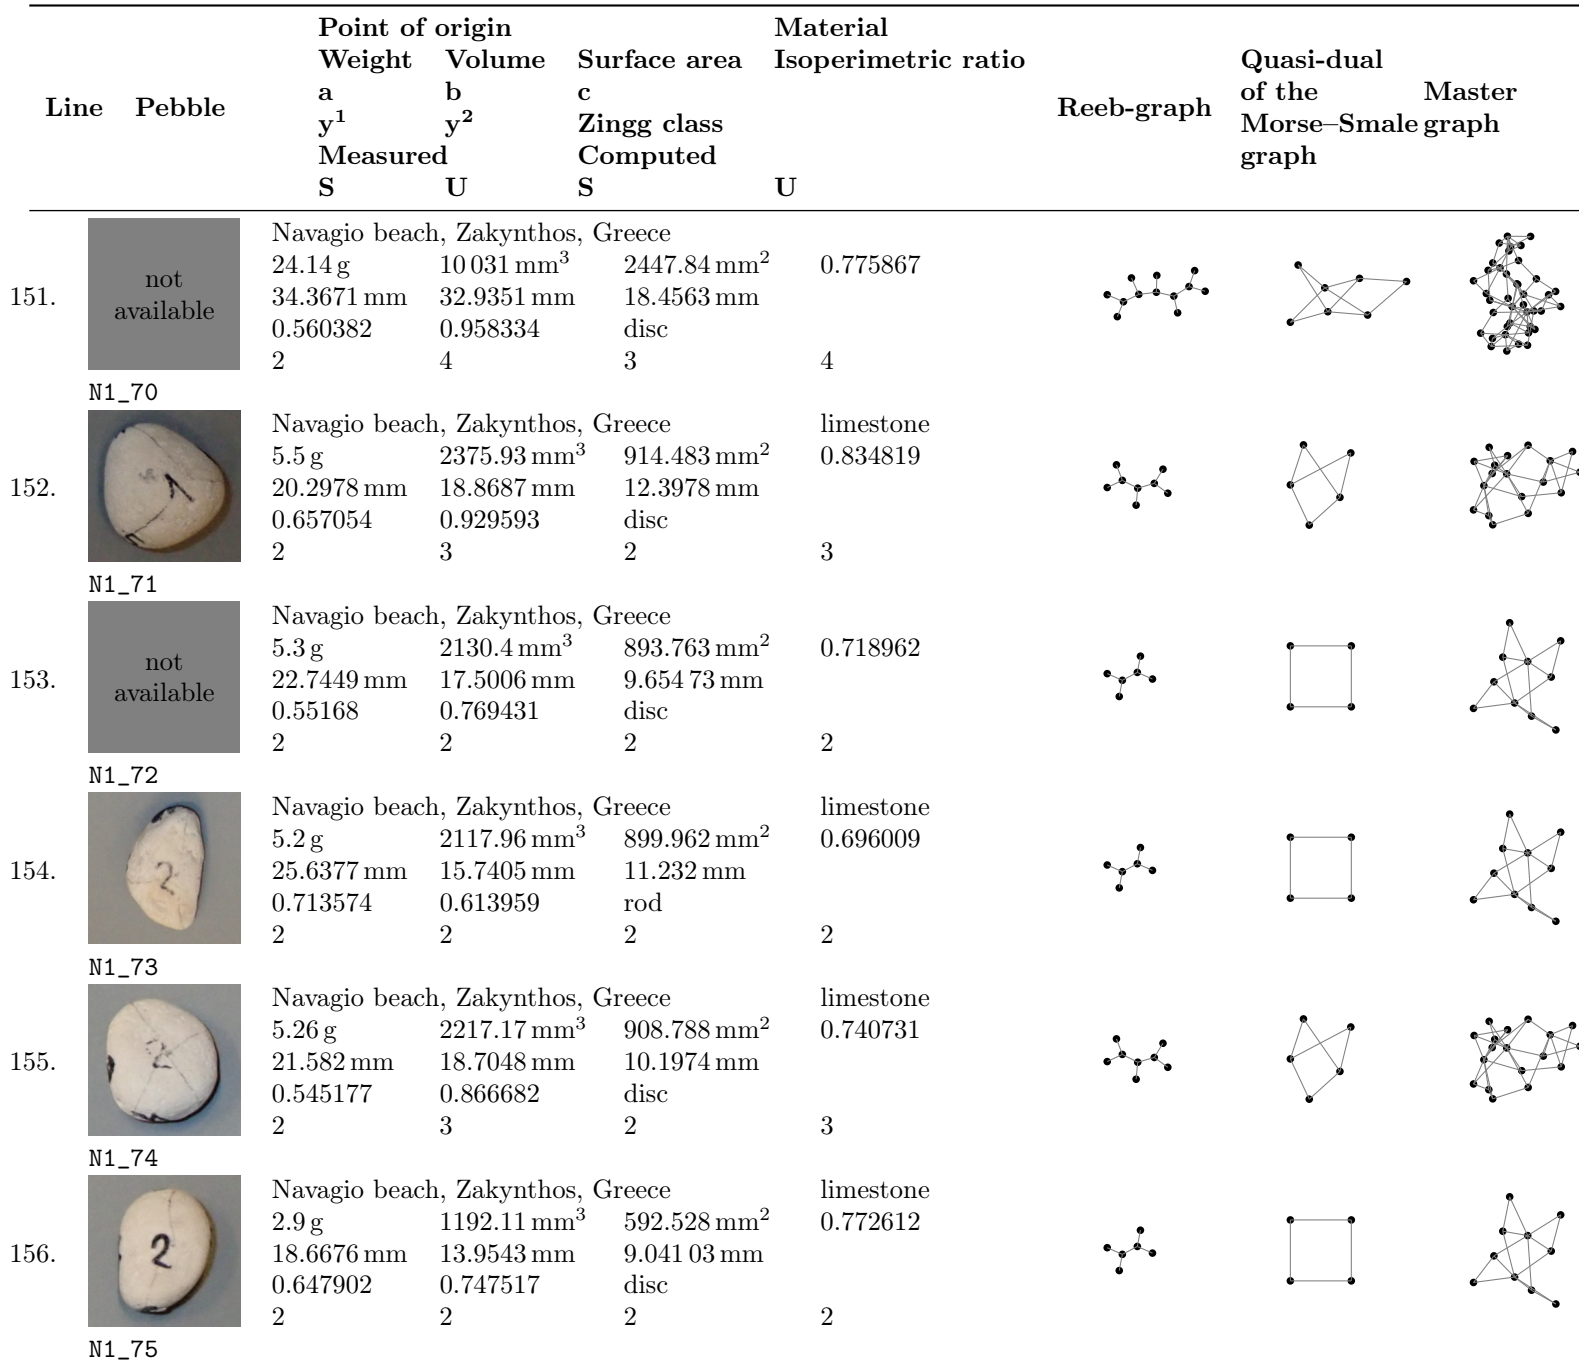   | Navagio beach, Zakynthos, Greece |                         |                         | limestone<br>0.834819 | 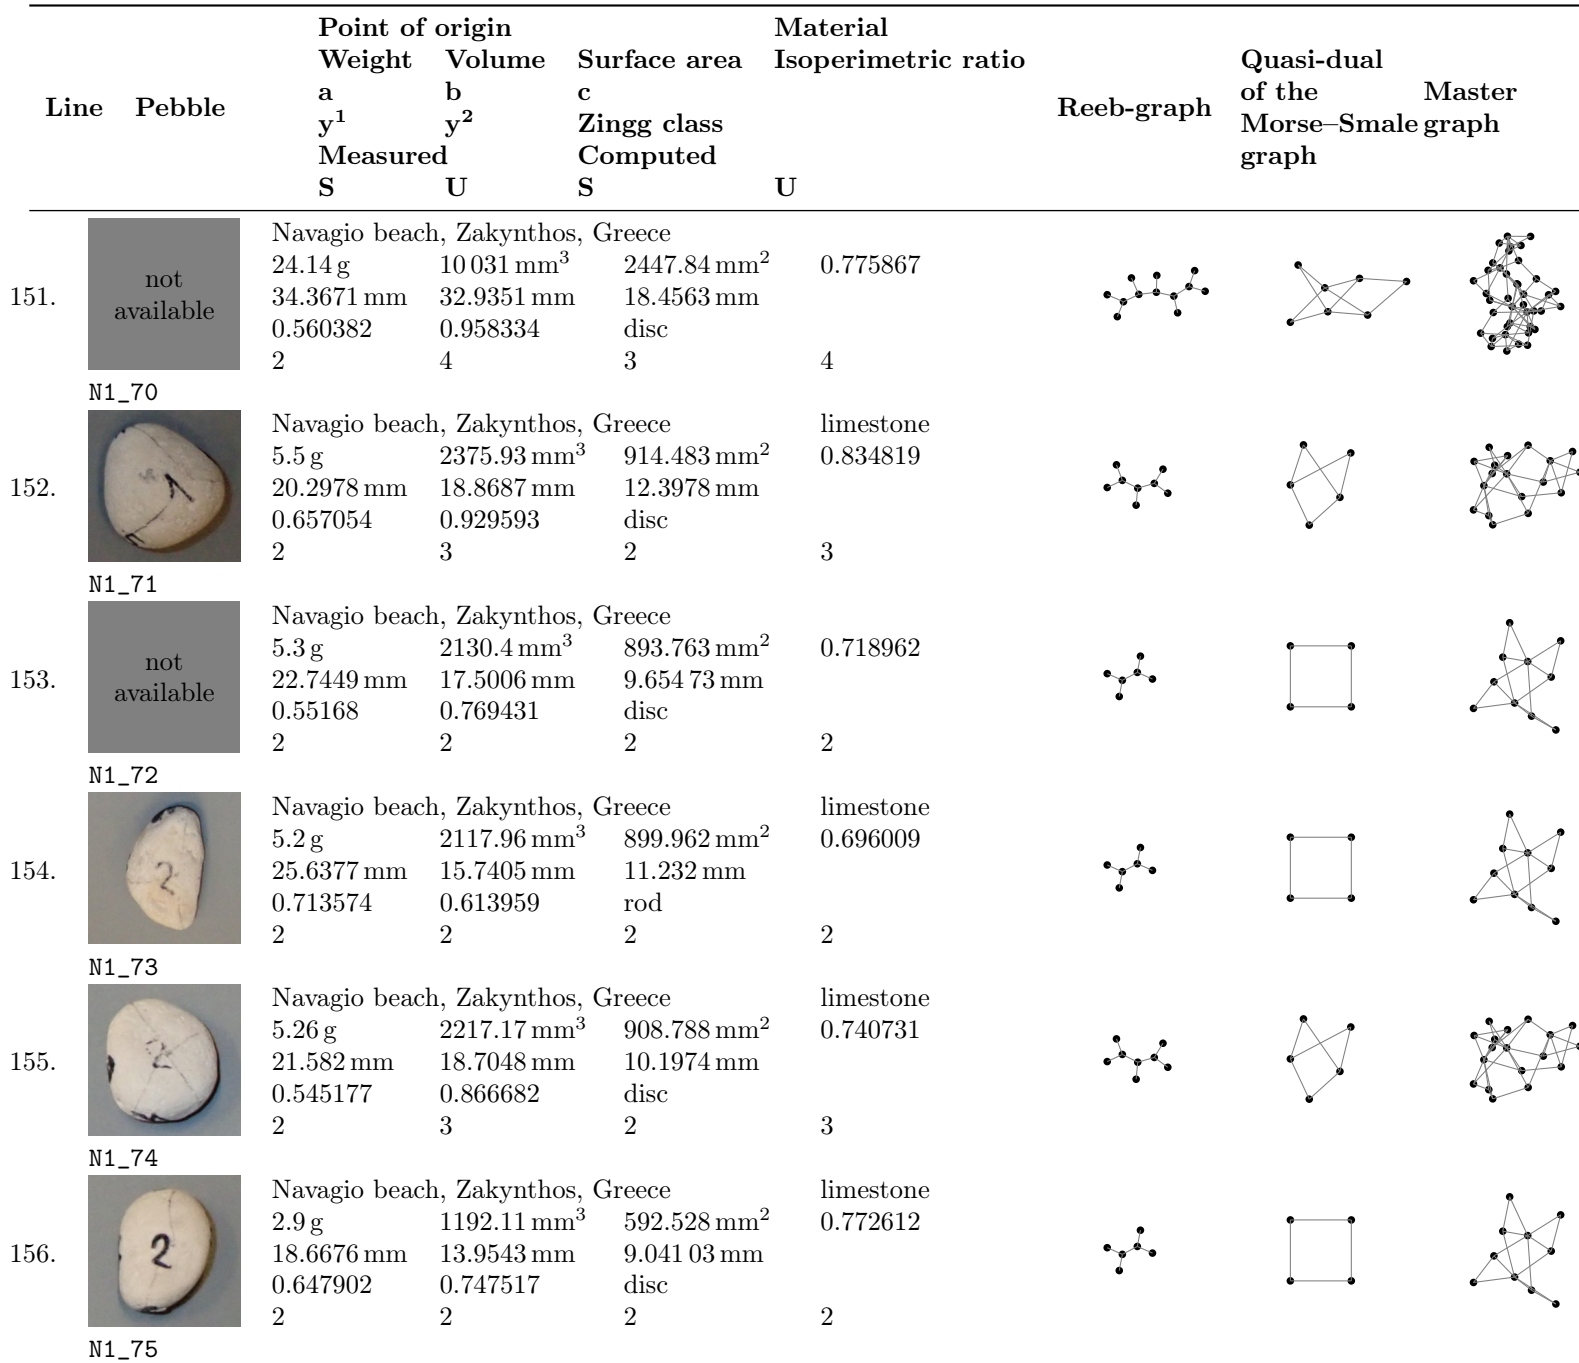   | 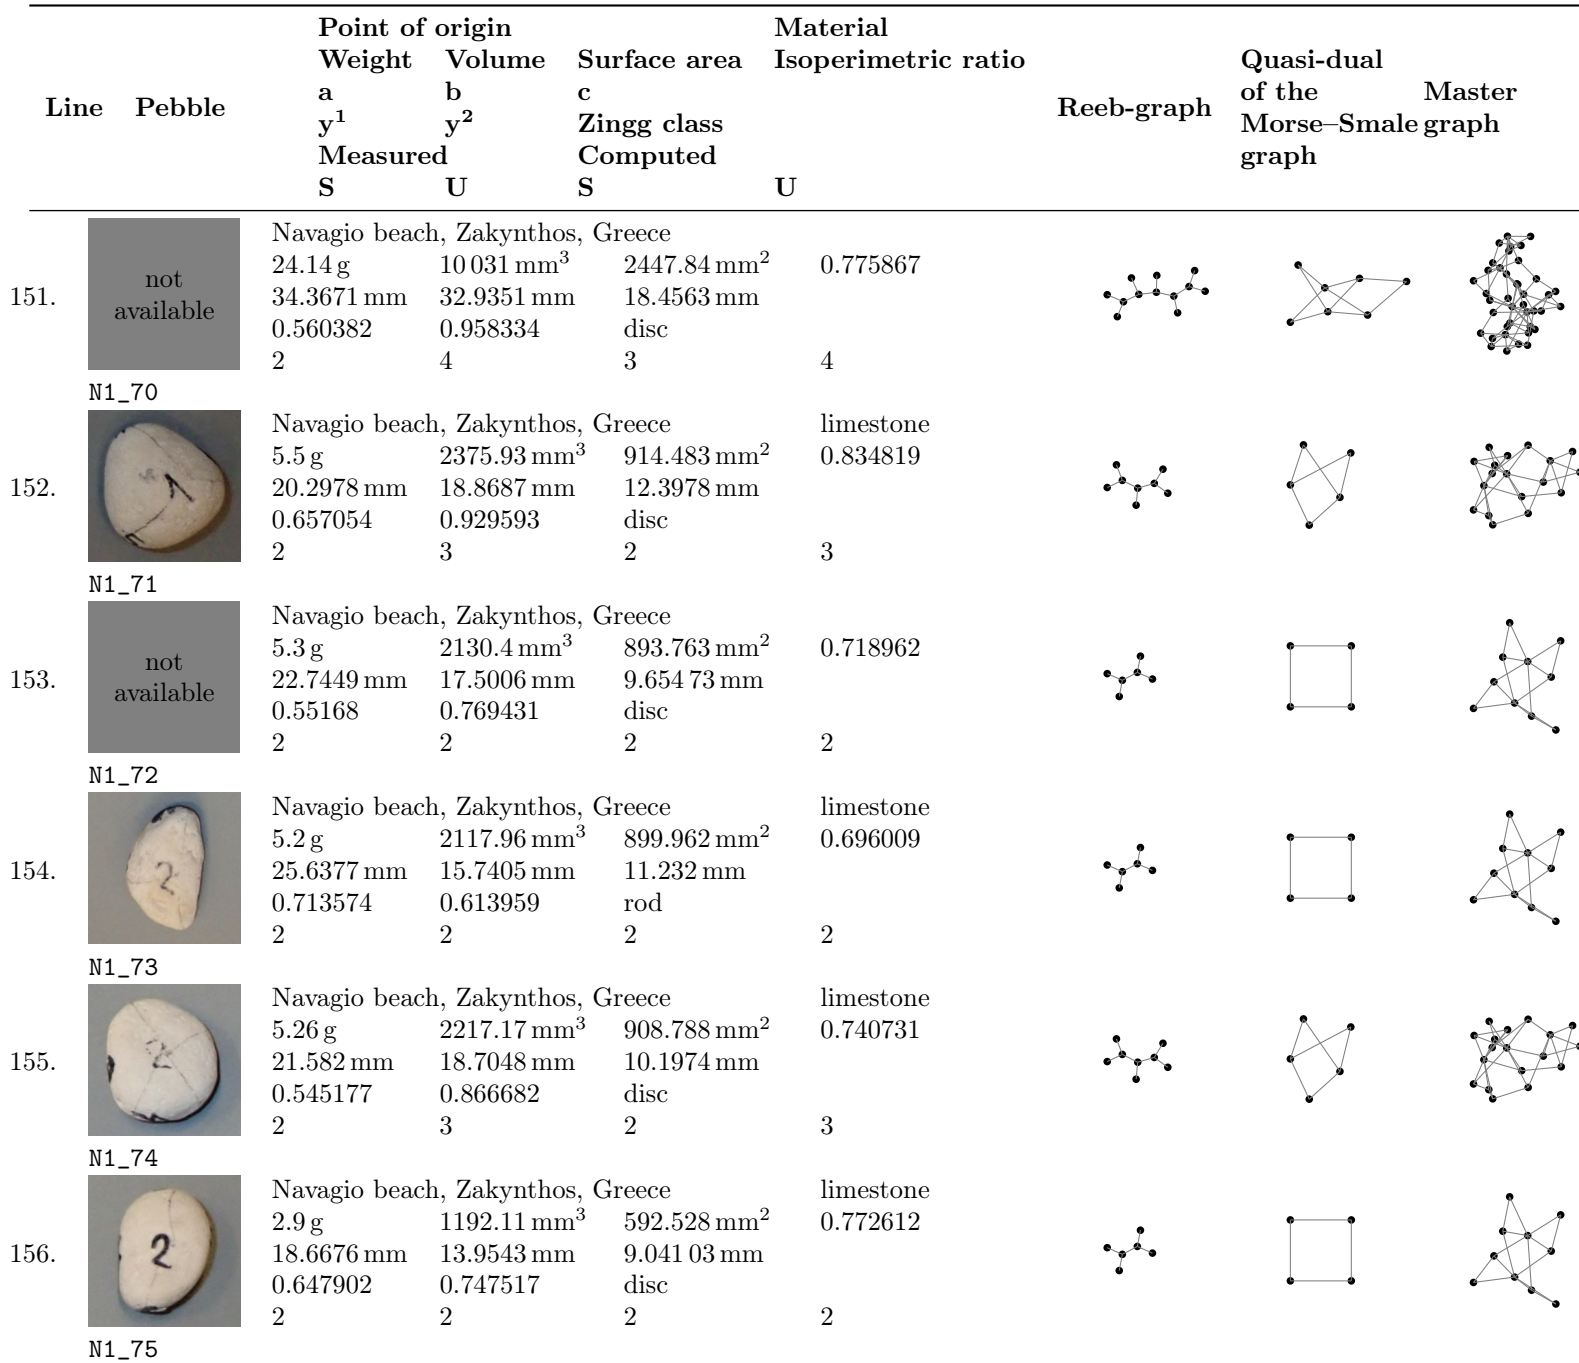   | 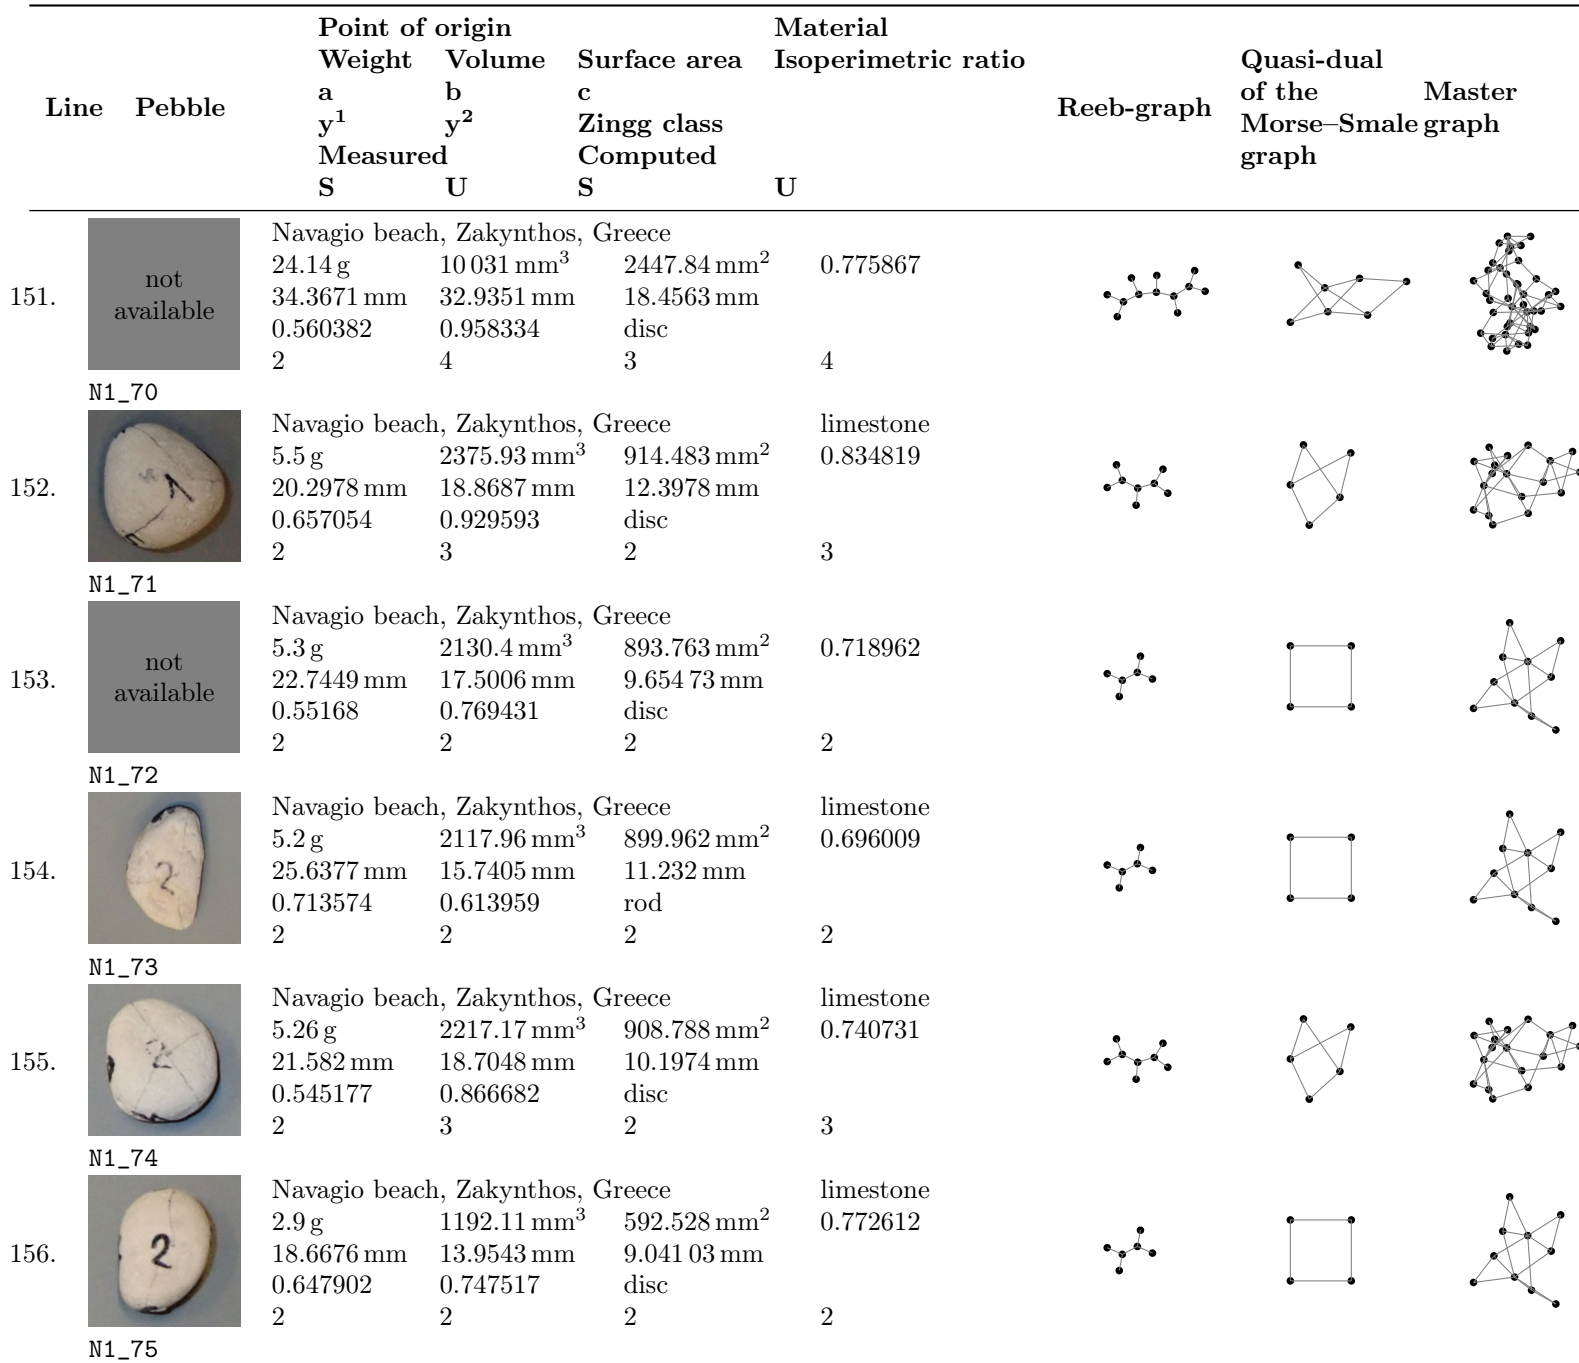   |
|      |                                                                                     | 5.5 g                            | 2375.93 mm <sup>3</sup> | 914.483 mm <sup>2</sup> |                       |                                                                                       |                                                                                       |                                                                                       |
|      |                                                                                     | 20.2978 mm                       | 18.8687 mm              | 12.3978 mm              |                       |                                                                                       |                                                                                       |                                                                                       |
|      |                                                                                     | 0.657054                         | 0.929593                | disc                    |                       |                                                                                       |                                                                                       |                                                                                       |
|      |                                                                                     | 2                                | 3                       | 2                       |                       |                                                                                       |                                                                                       |                                                                                       |
|      | N1_71                                                                               |                                  |                         |                         |                       |                                                                                       |                                                                                       |                                                                                       |
| 153. | 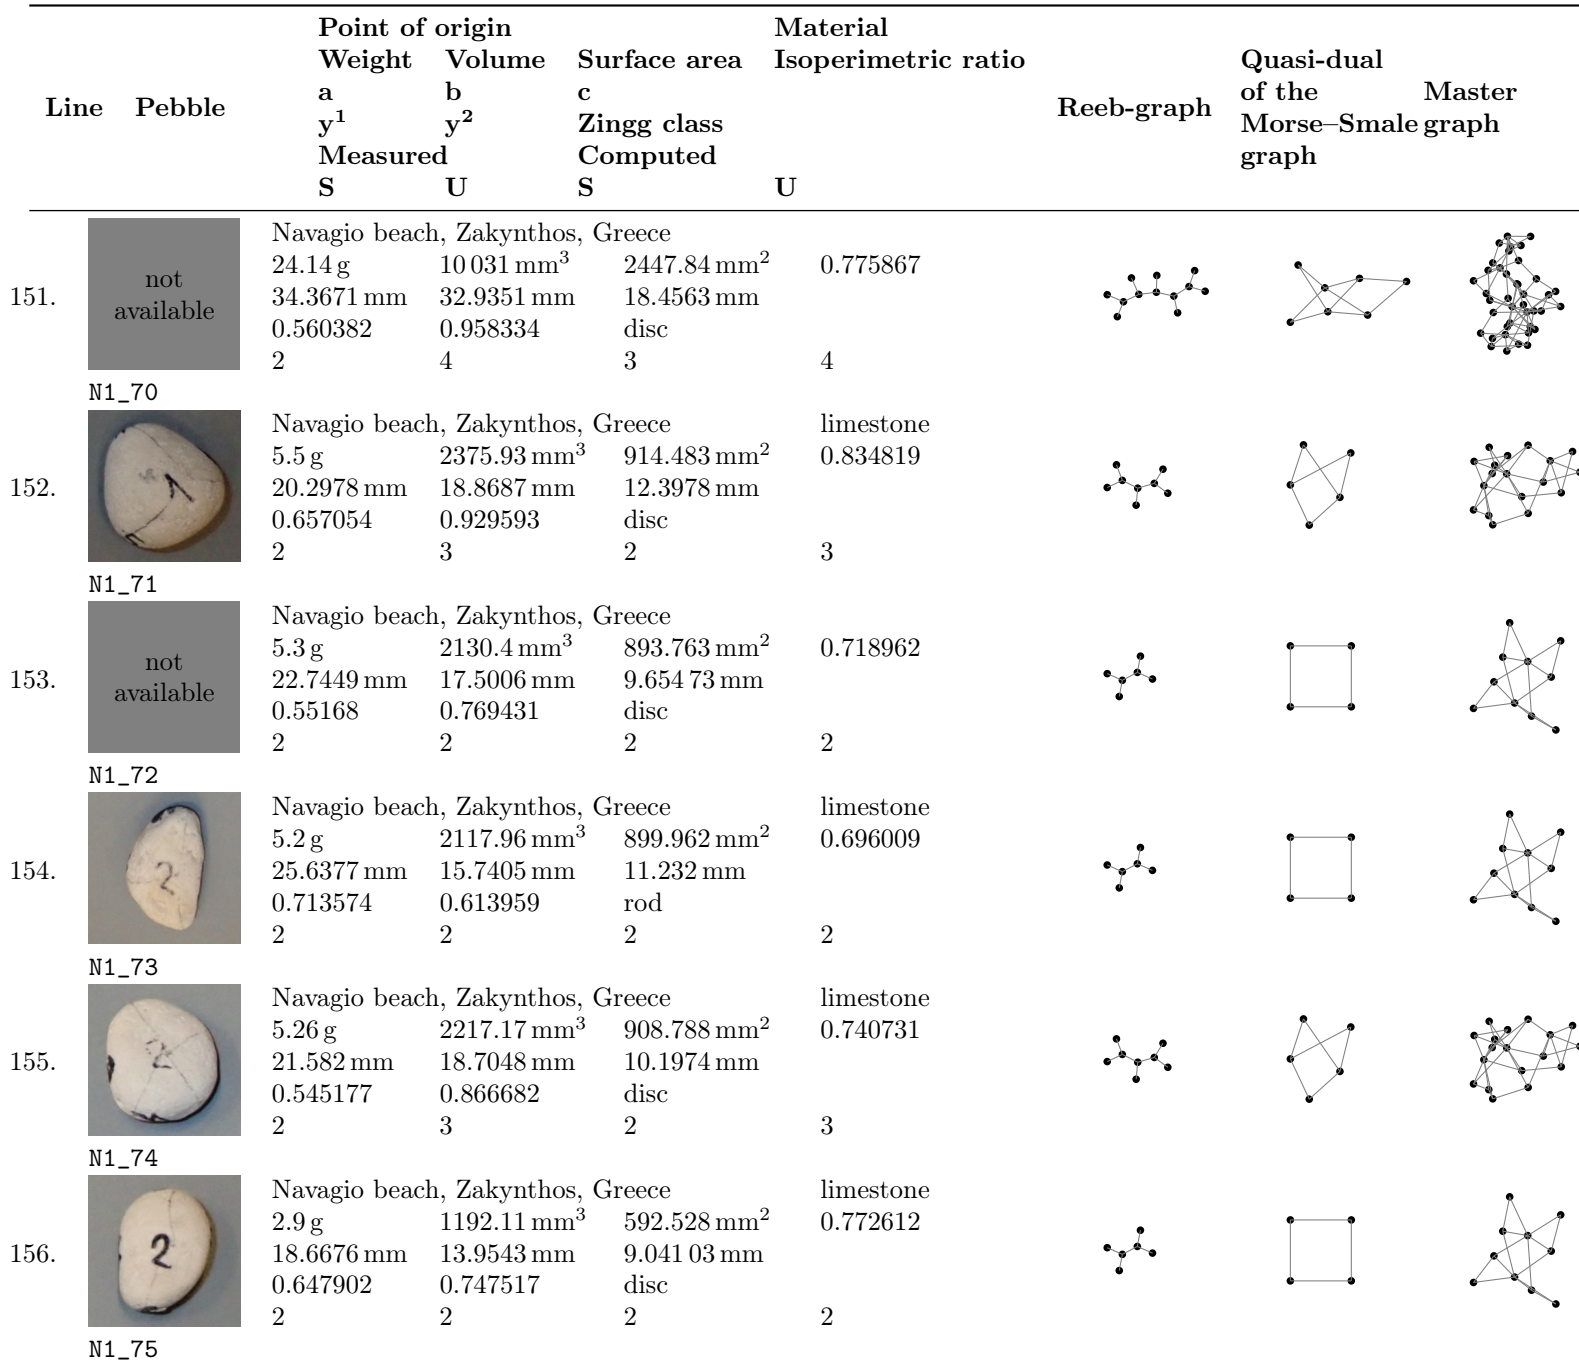   | Navagio beach, Zakynthos, Greece |                         |                         | 0.718962              | 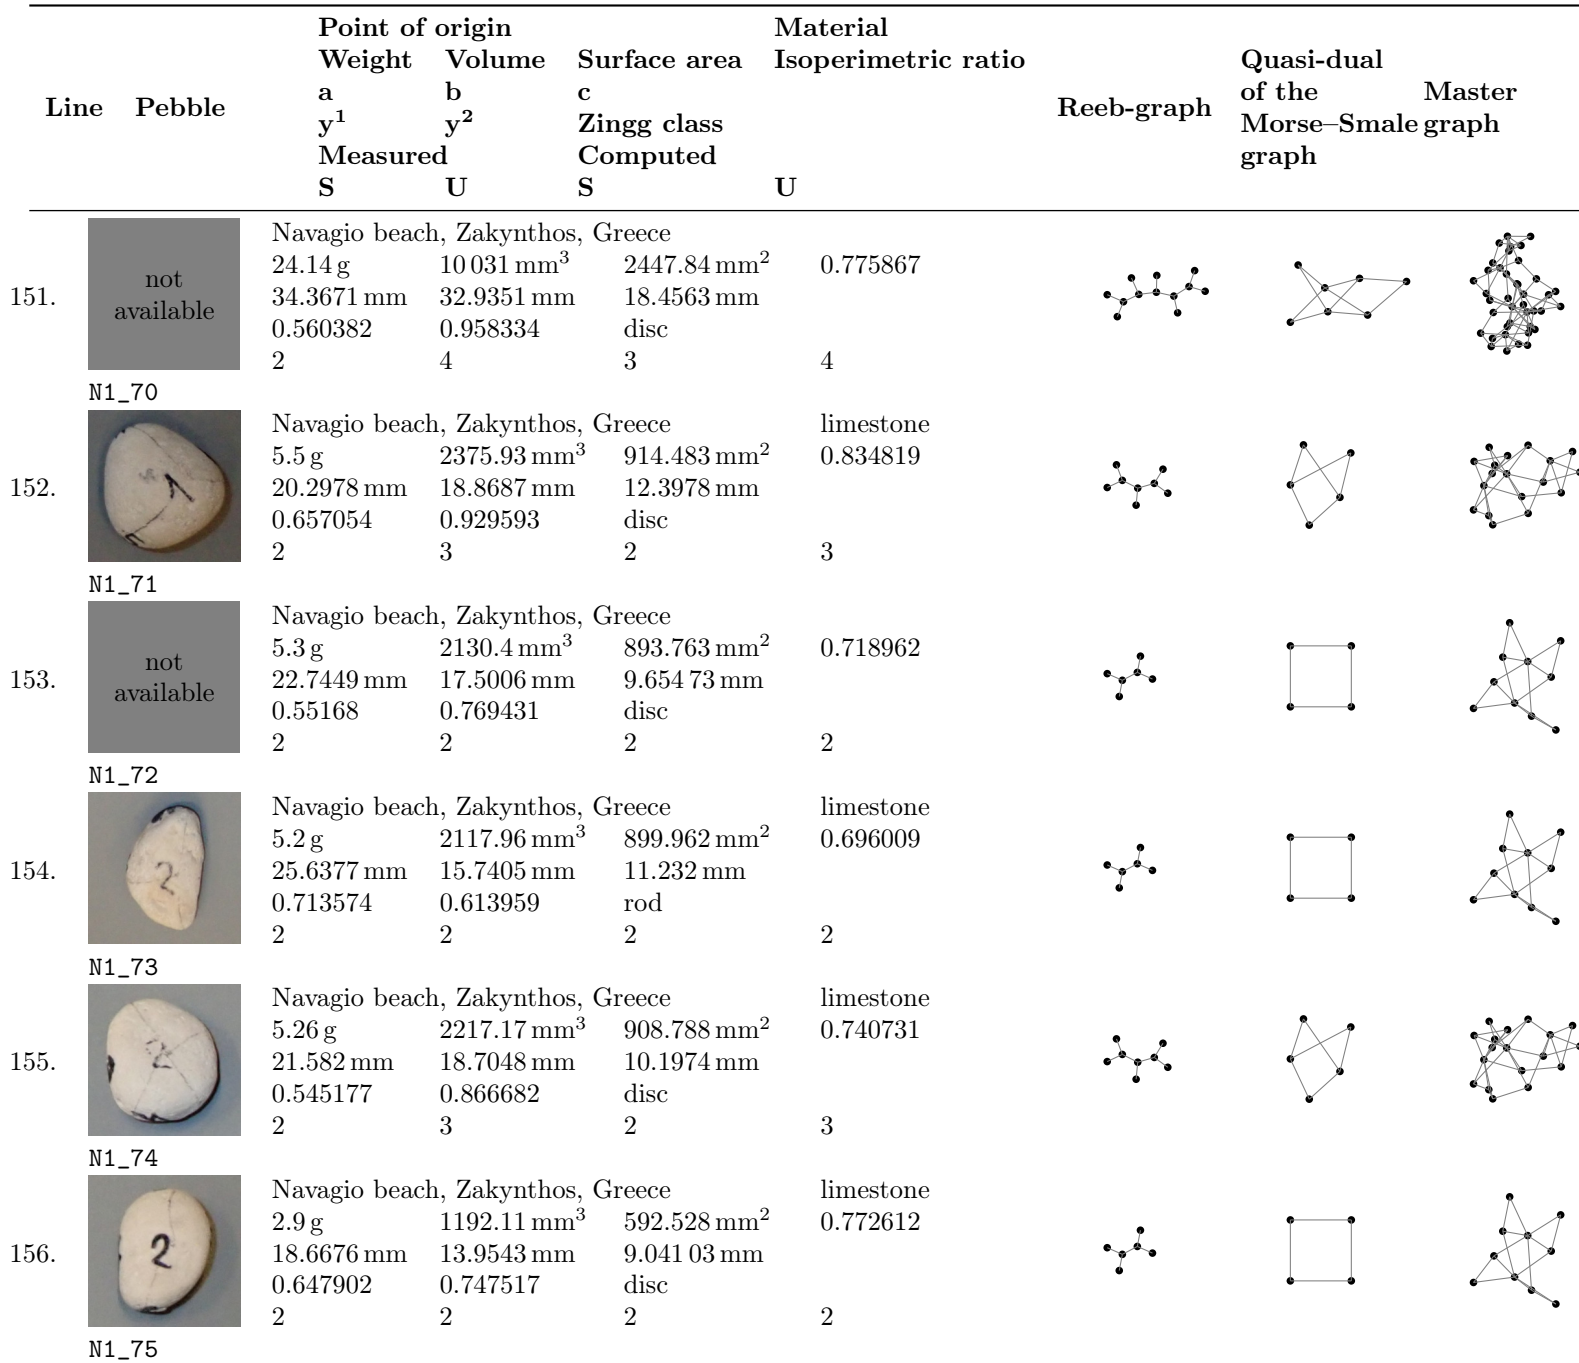   | 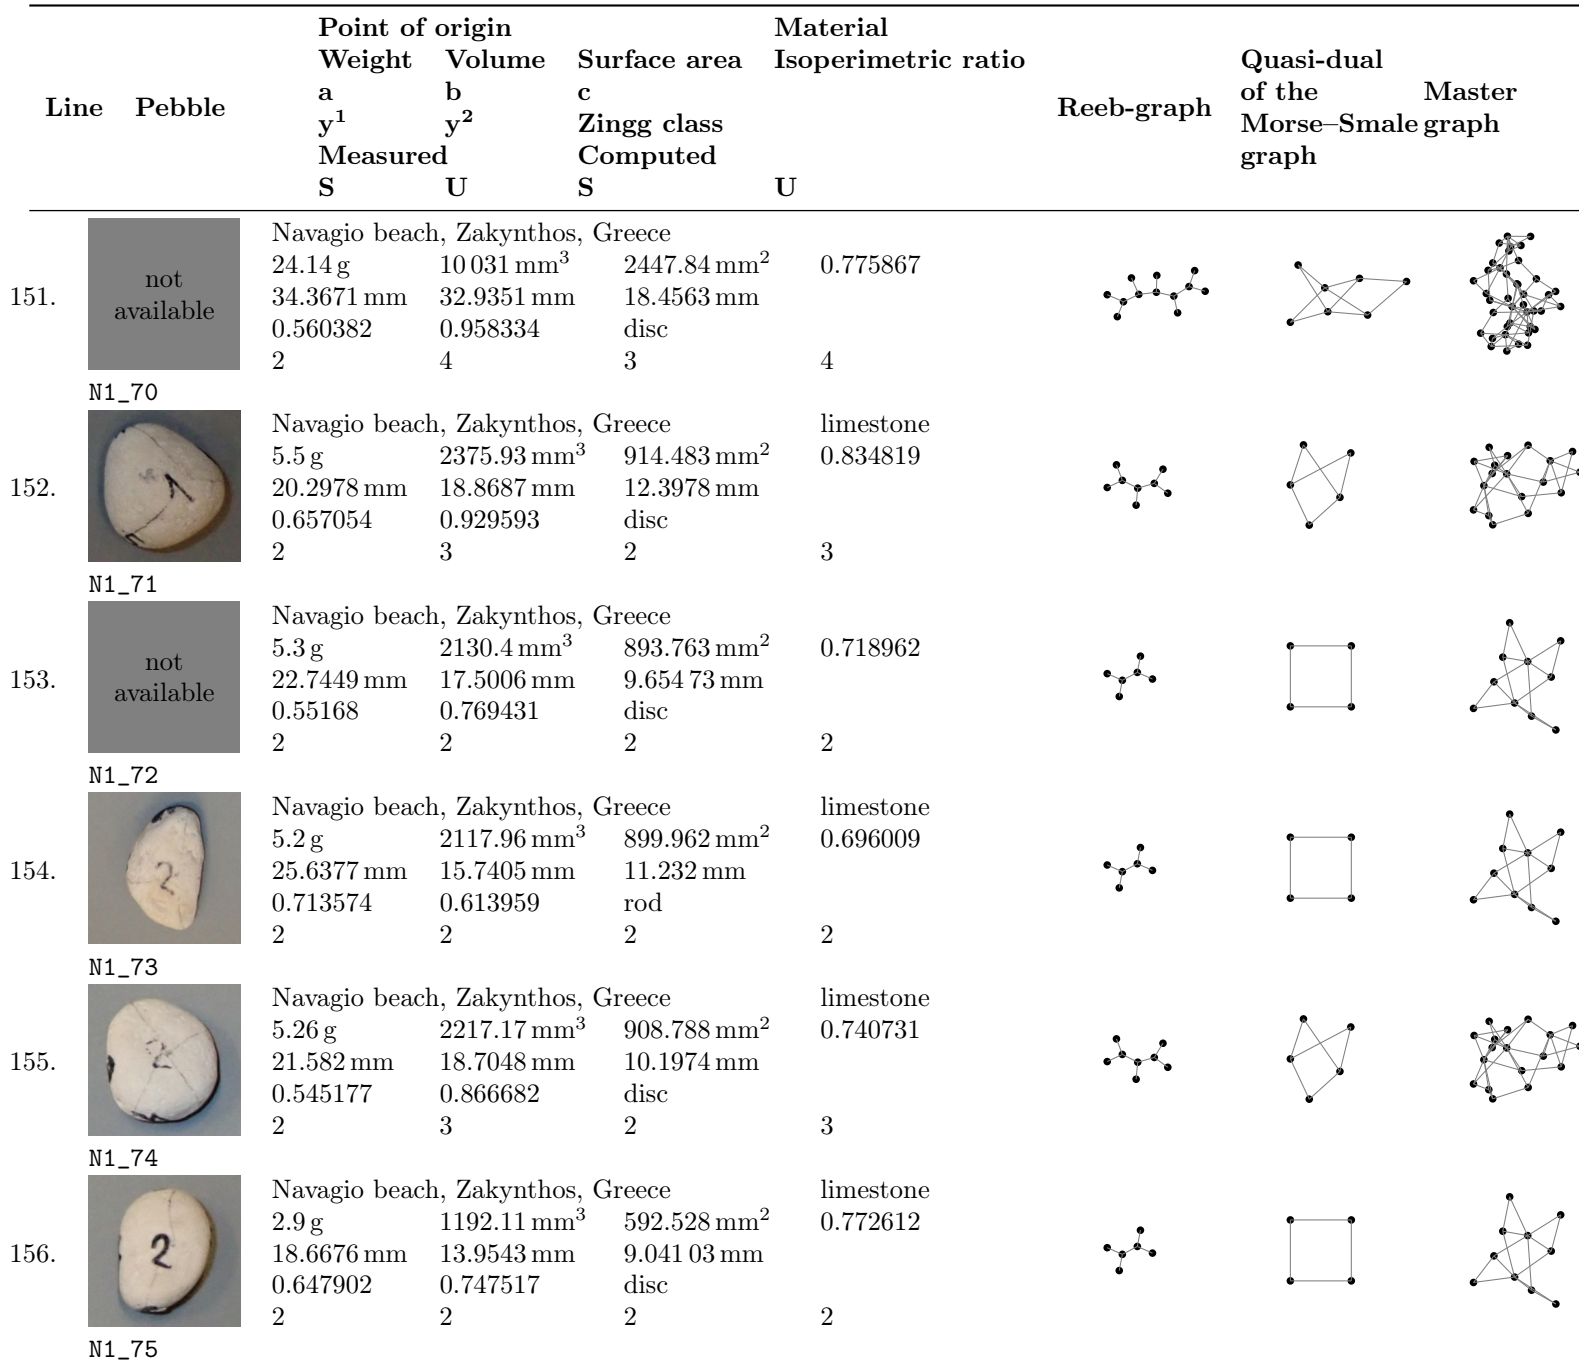   | 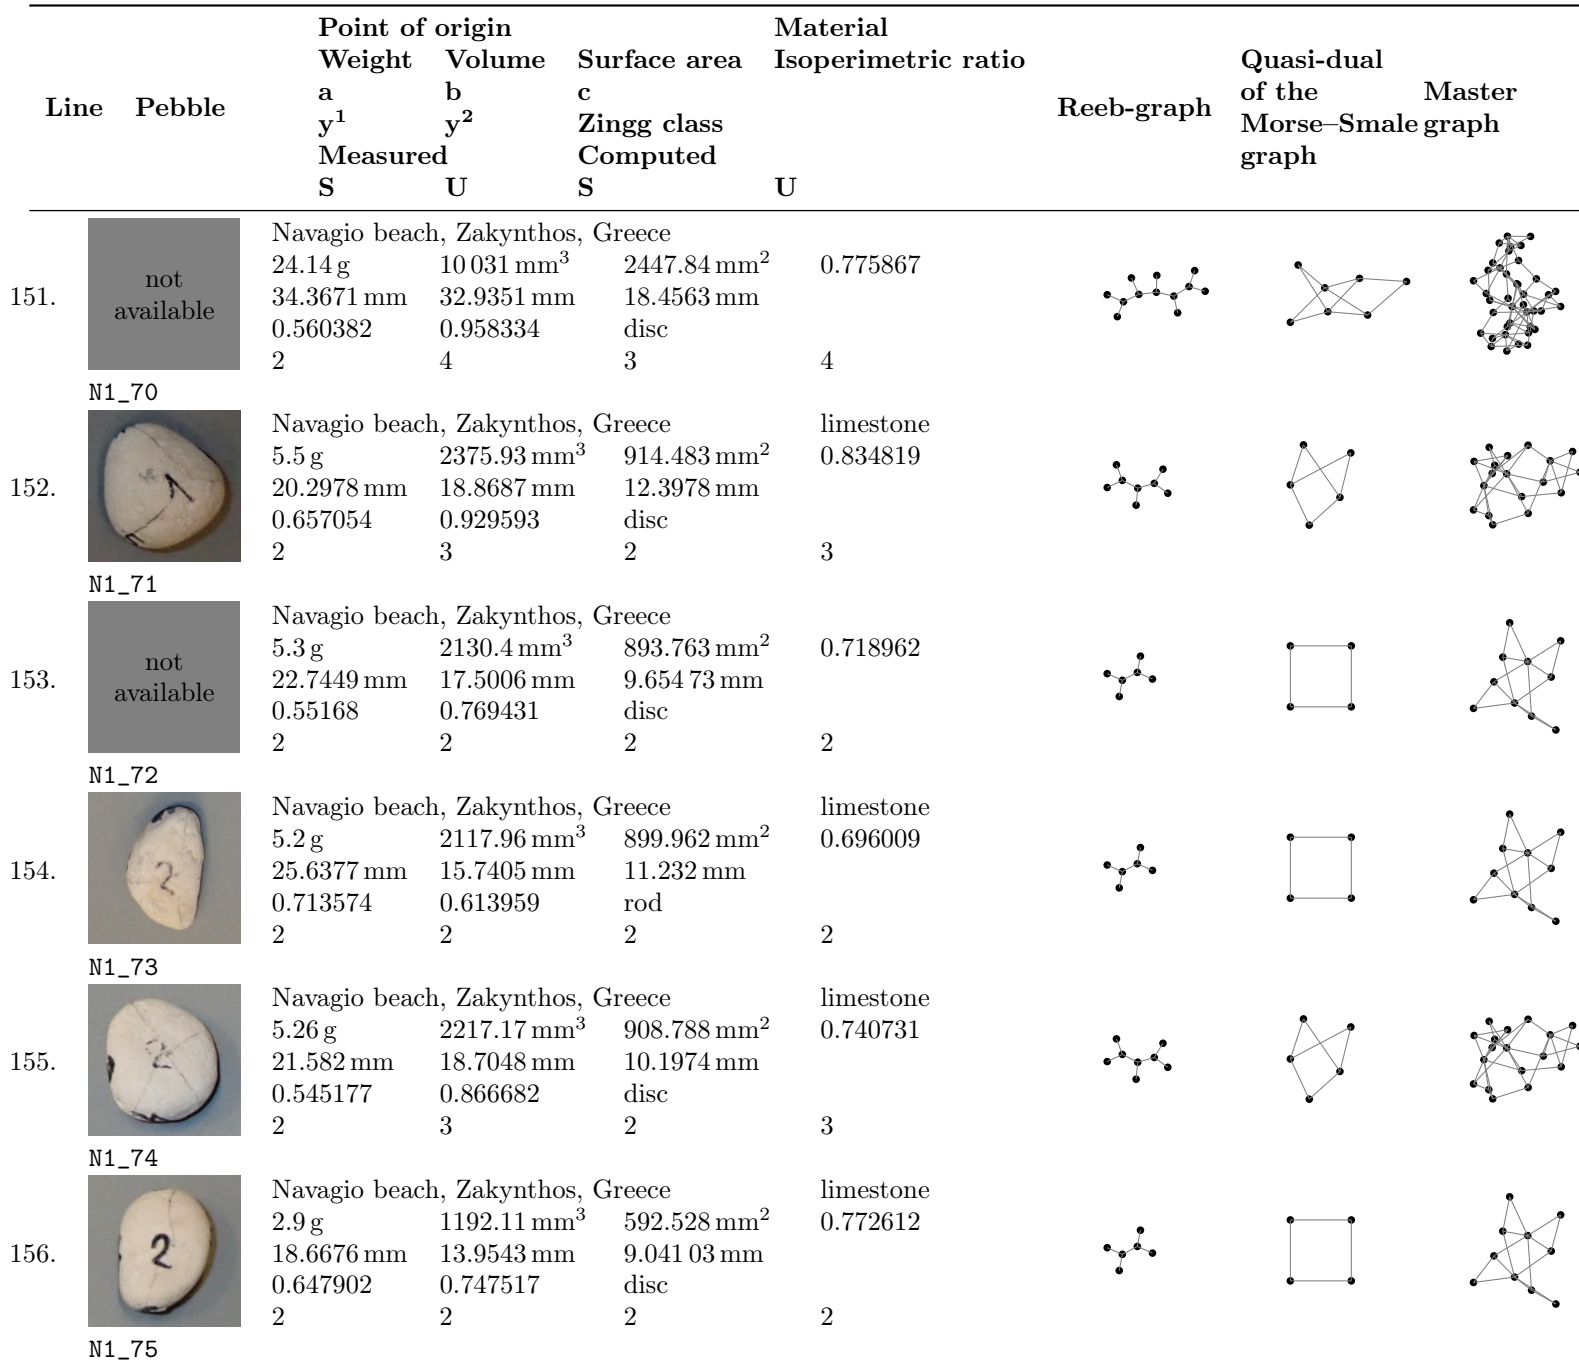   |
|      |                                                                                     | 5.3 g                            | 2130.4 mm <sup>3</sup>  | 893.763 mm <sup>2</sup> |                       |                                                                                       |                                                                                       |                                                                                       |
|      |                                                                                     | 22.7449 mm                       | 17.5006 mm              | 9.654 73 mm             |                       |                                                                                       |                                                                                       |                                                                                       |
|      |                                                                                     | 0.55168                          | 0.769431                | disc                    |                       |                                                                                       |                                                                                       |                                                                                       |
|      |                                                                                     | 2                                | 2                       | 2                       |                       |                                                                                       |                                                                                       |                                                                                       |
|      | N1_72                                                                               |                                  |                         |                         |                       |                                                                                       |                                                                                       |                                                                                       |
| 154. | 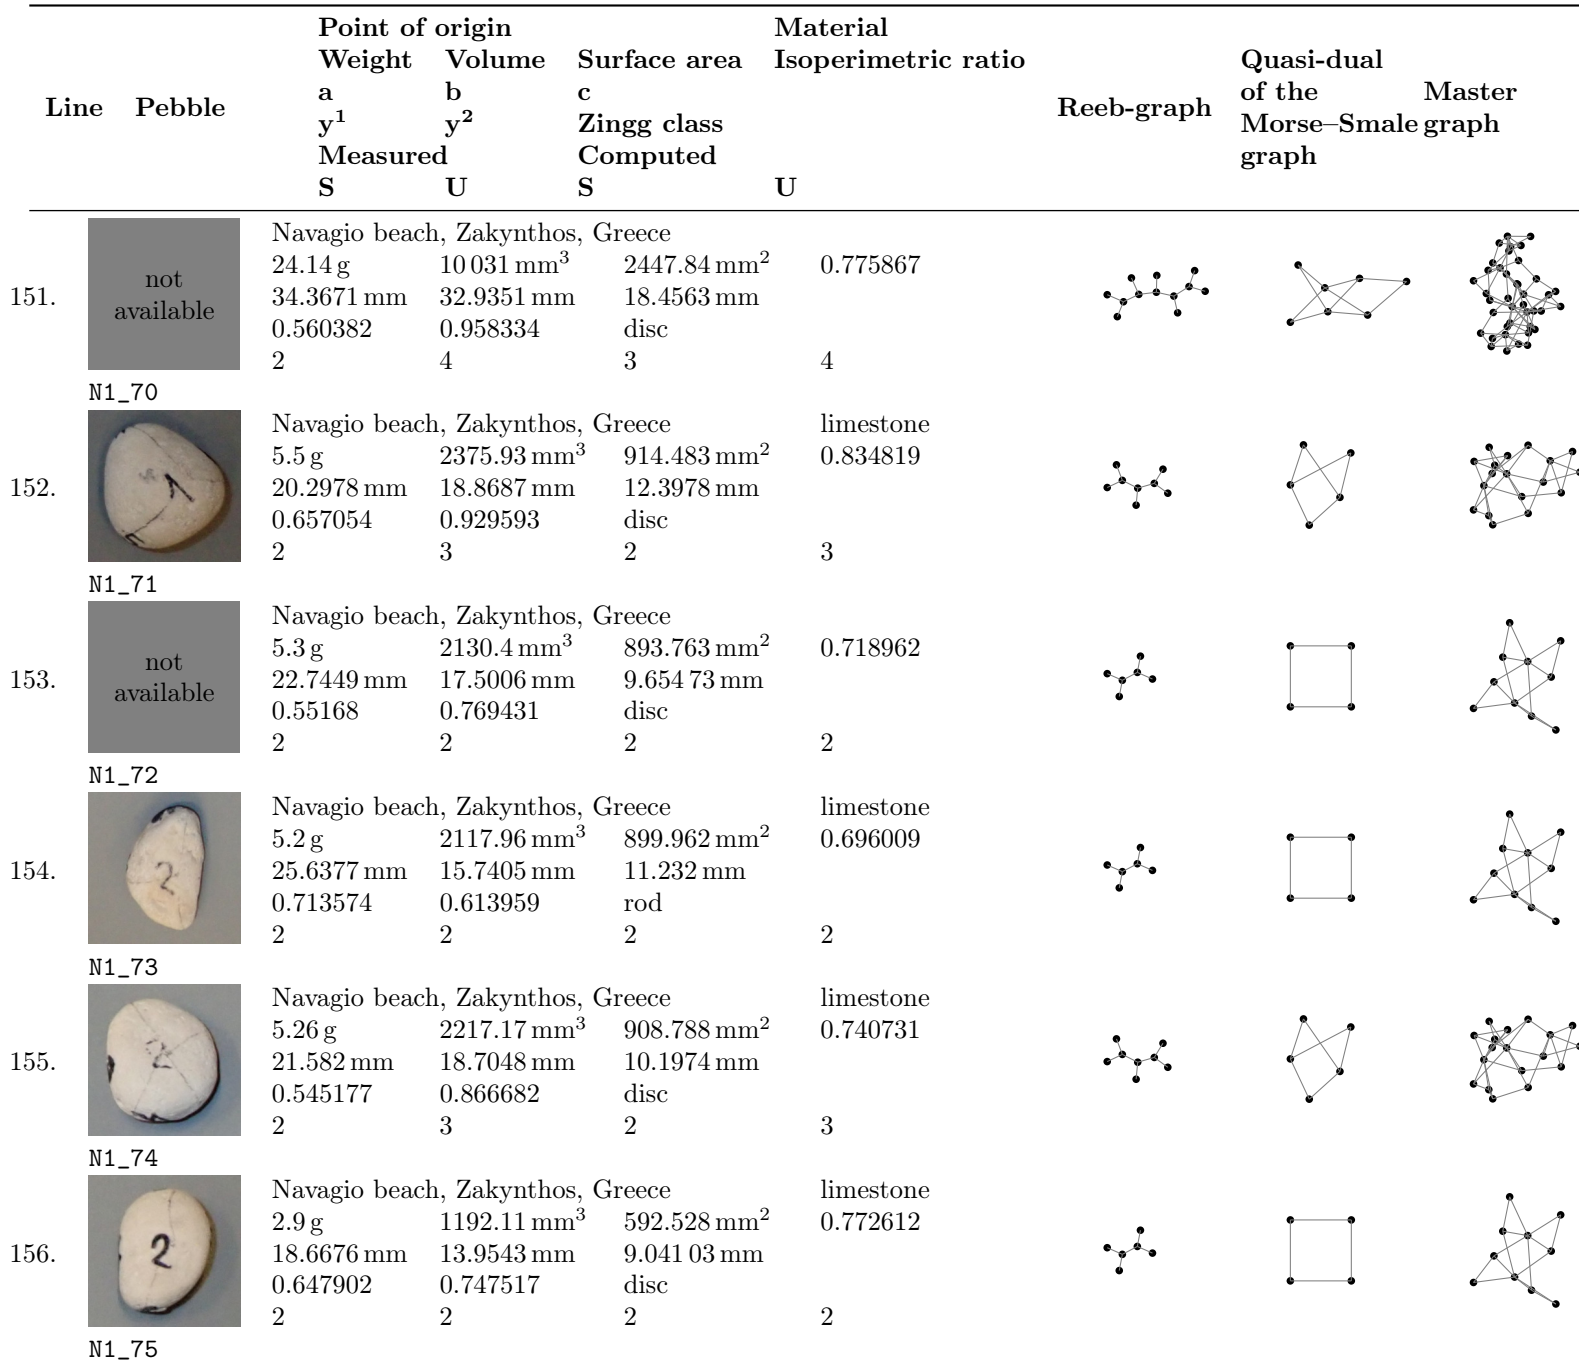  | Navagio beach, Zakynthos, Greece |                         |                         | limestone<br>0.696009 | 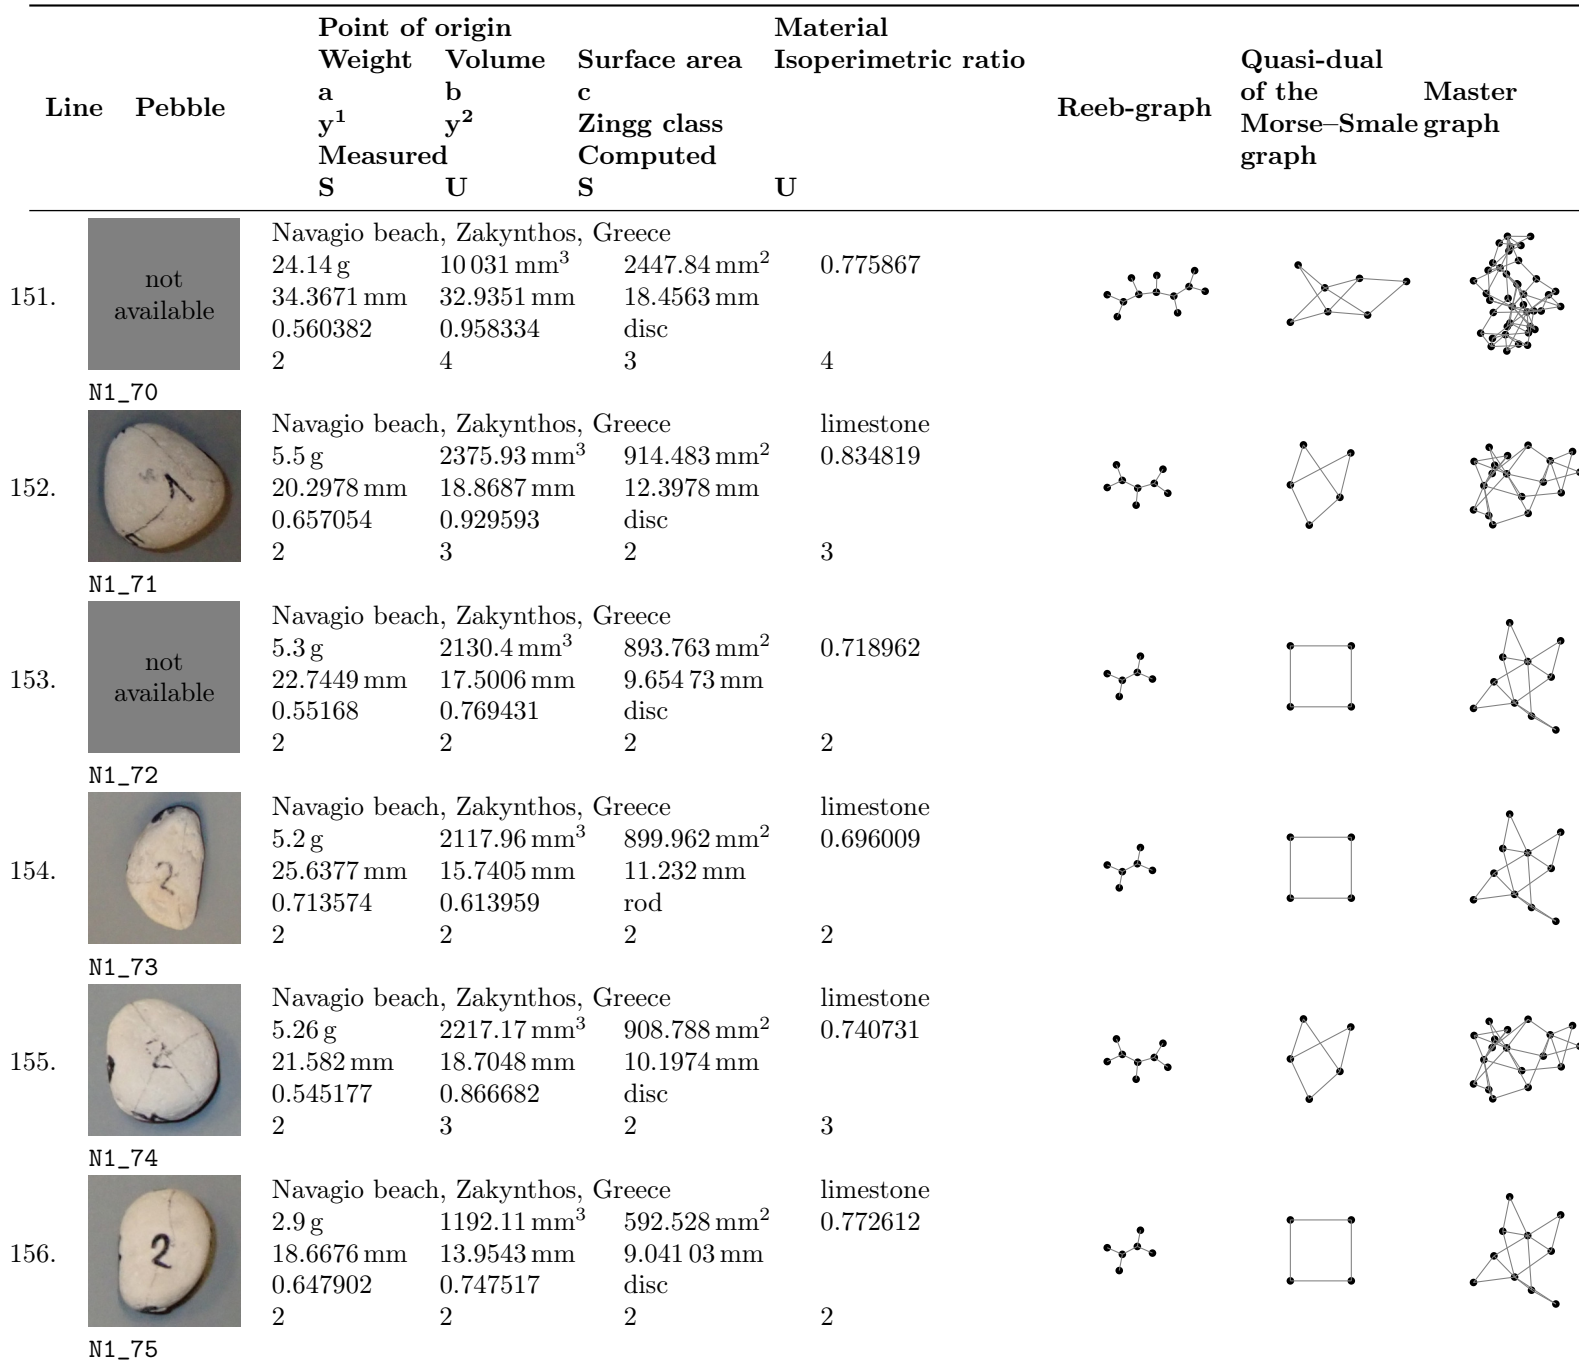  | 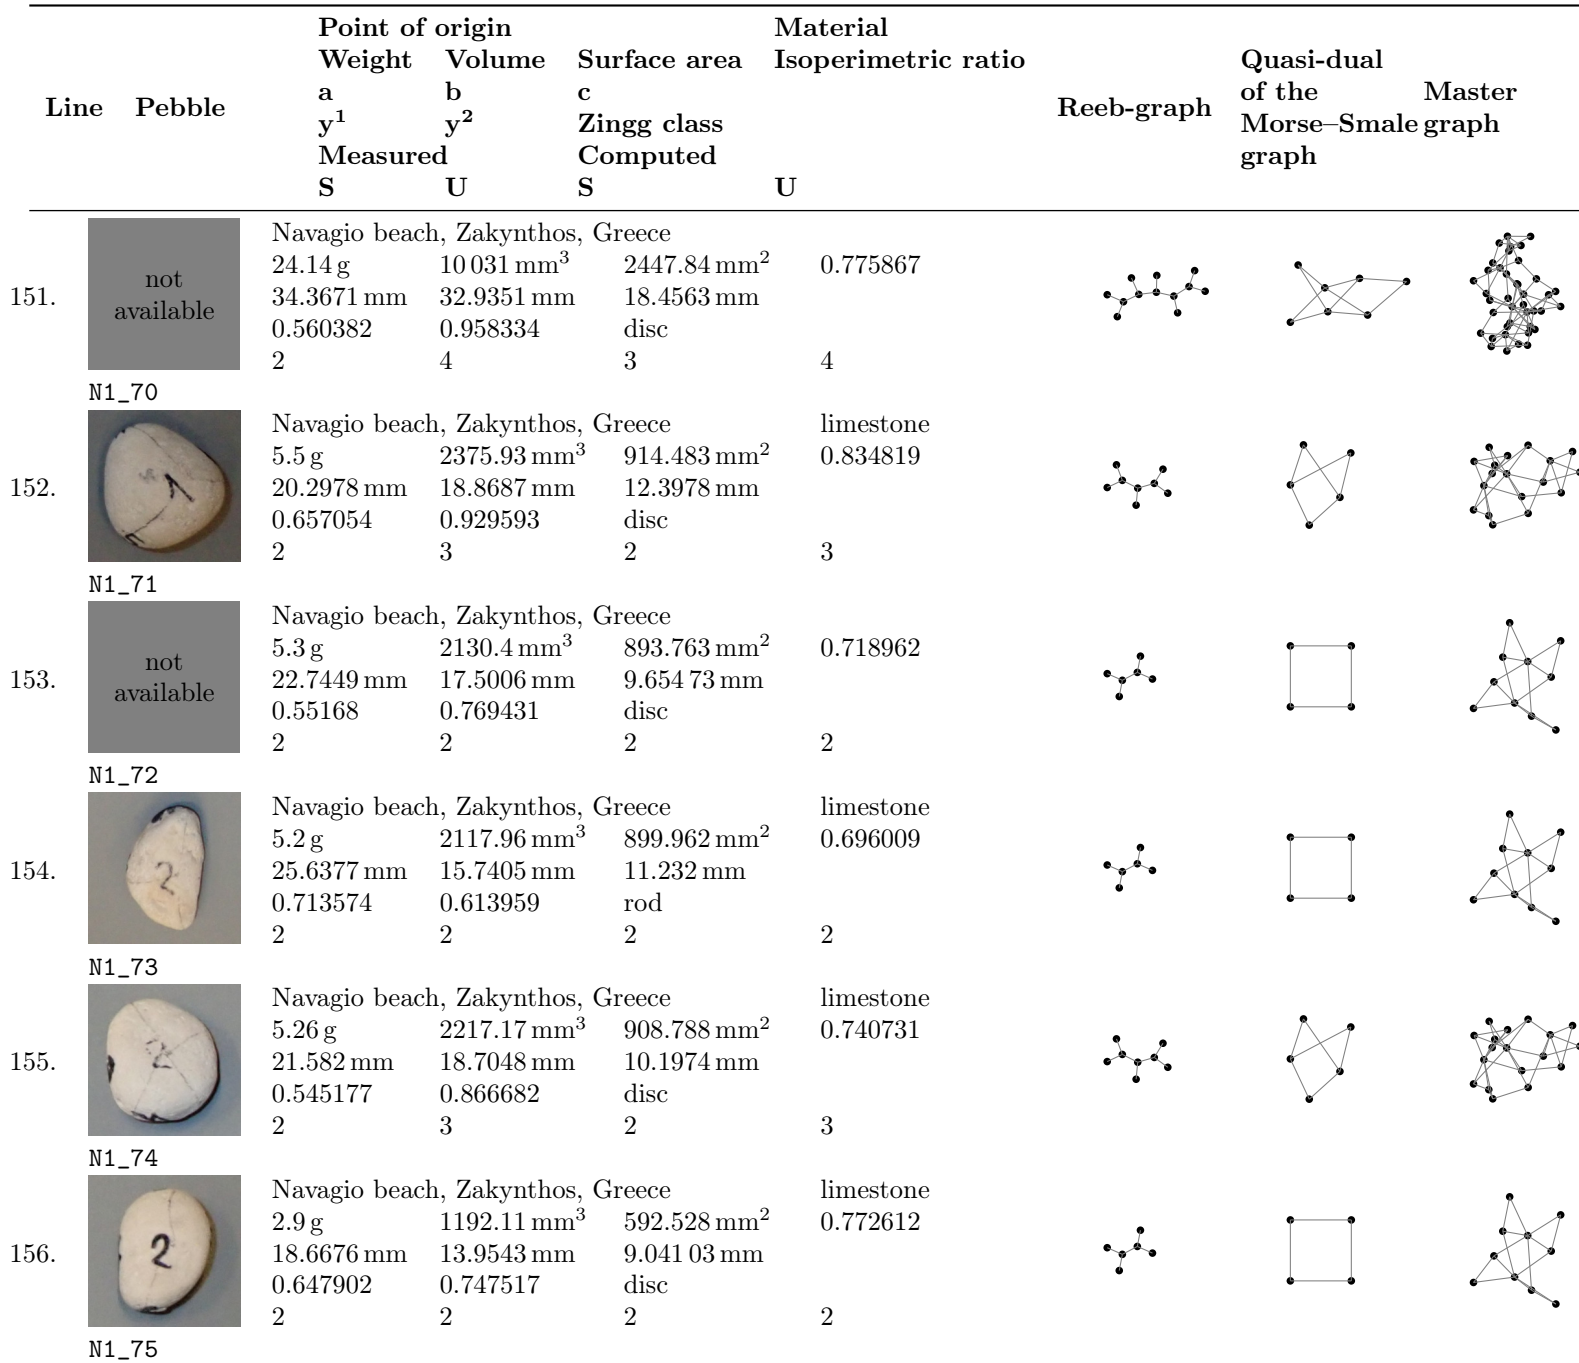  | 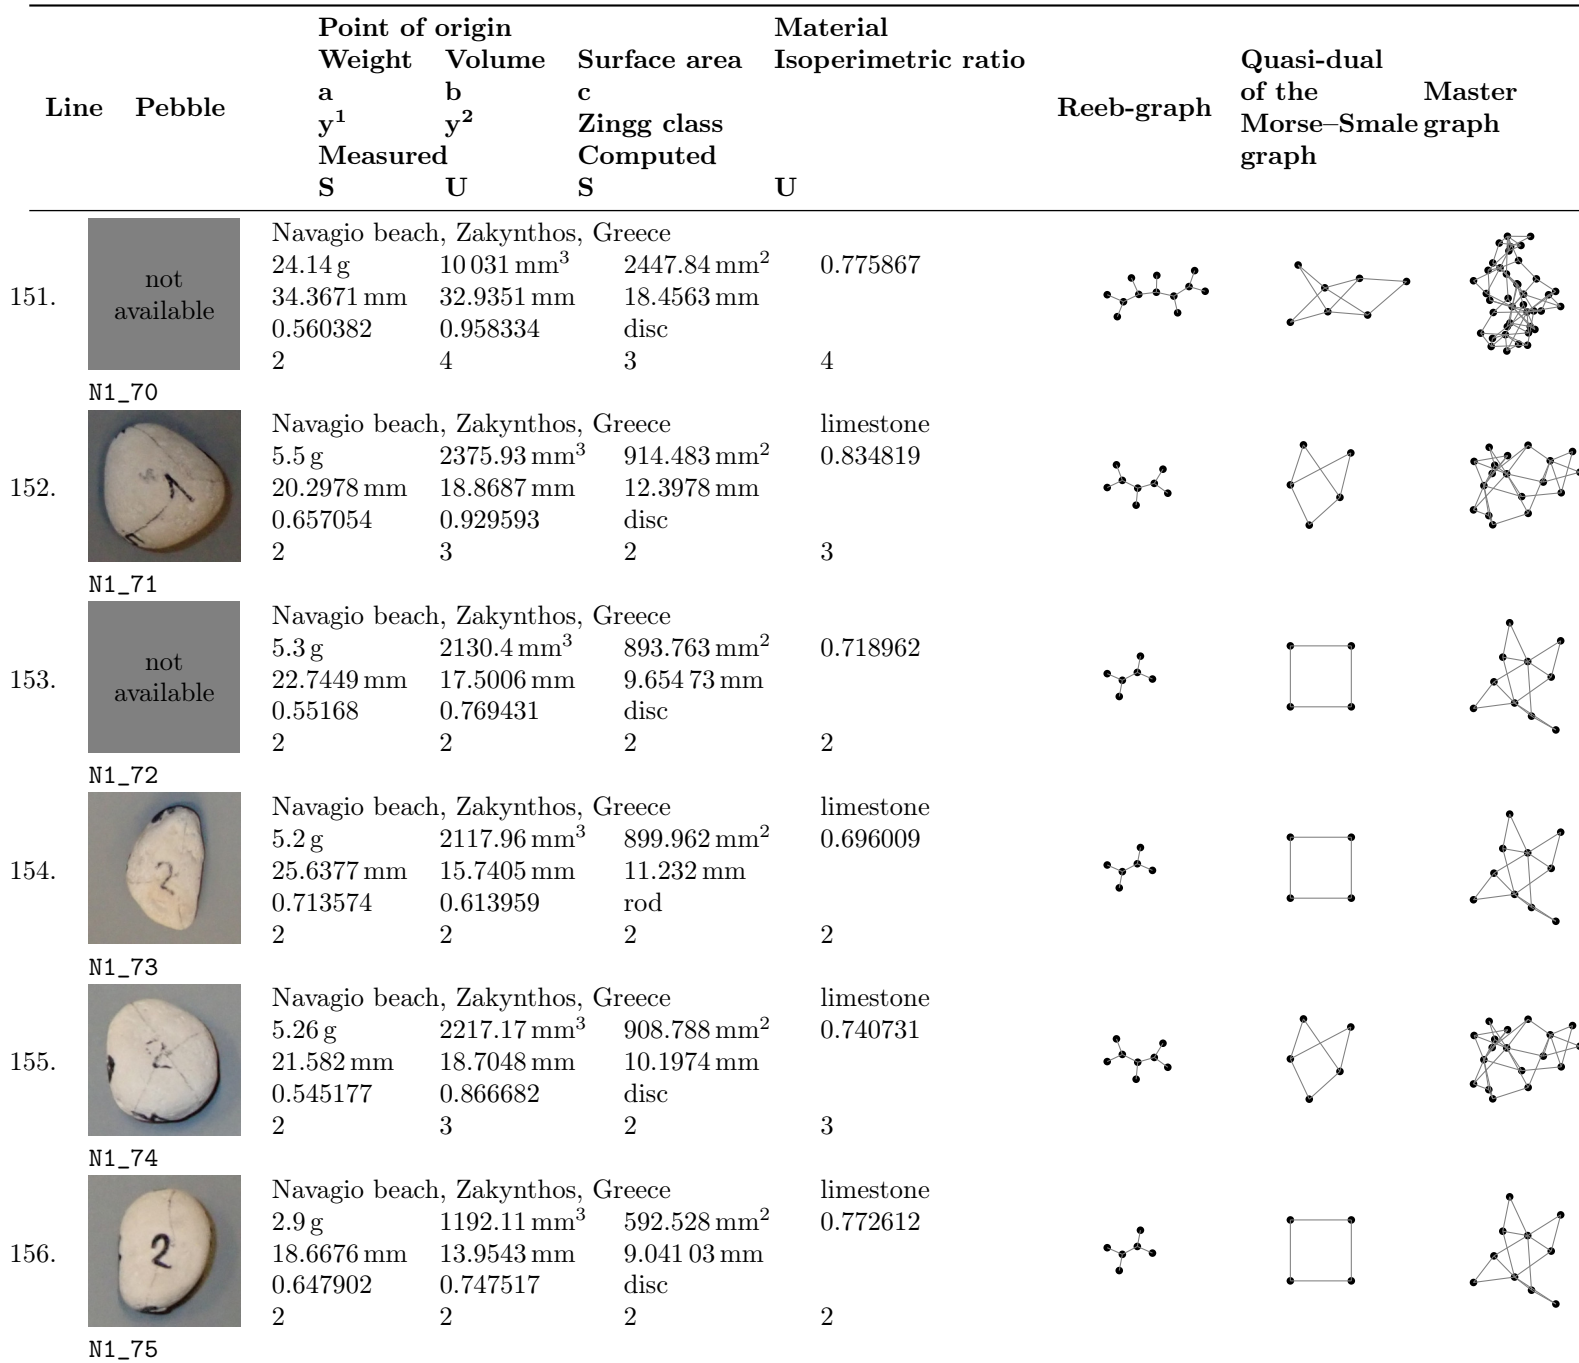  |
|      |                                                                                     | 5.2 g                            | 2117.96 mm <sup>3</sup> | 899.962 mm <sup>2</sup> |                       |                                                                                       |                                                                                       |                                                                                       |
|      |                                                                                     | 25.6377 mm                       | 15.7405 mm              | 11.232 mm               |                       |                                                                                       |                                                                                       |                                                                                       |
|      |                                                                                     | 0.713574                         | 0.613959                | rod                     |                       |                                                                                       |                                                                                       |                                                                                       |
|      |                                                                                     | 2                                | 2                       | 2                       |                       |                                                                                       |                                                                                       |                                                                                       |
|      | N1_73                                                                               |                                  |                         |                         |                       |                                                                                       |                                                                                       |                                                                                       |
| 155. | 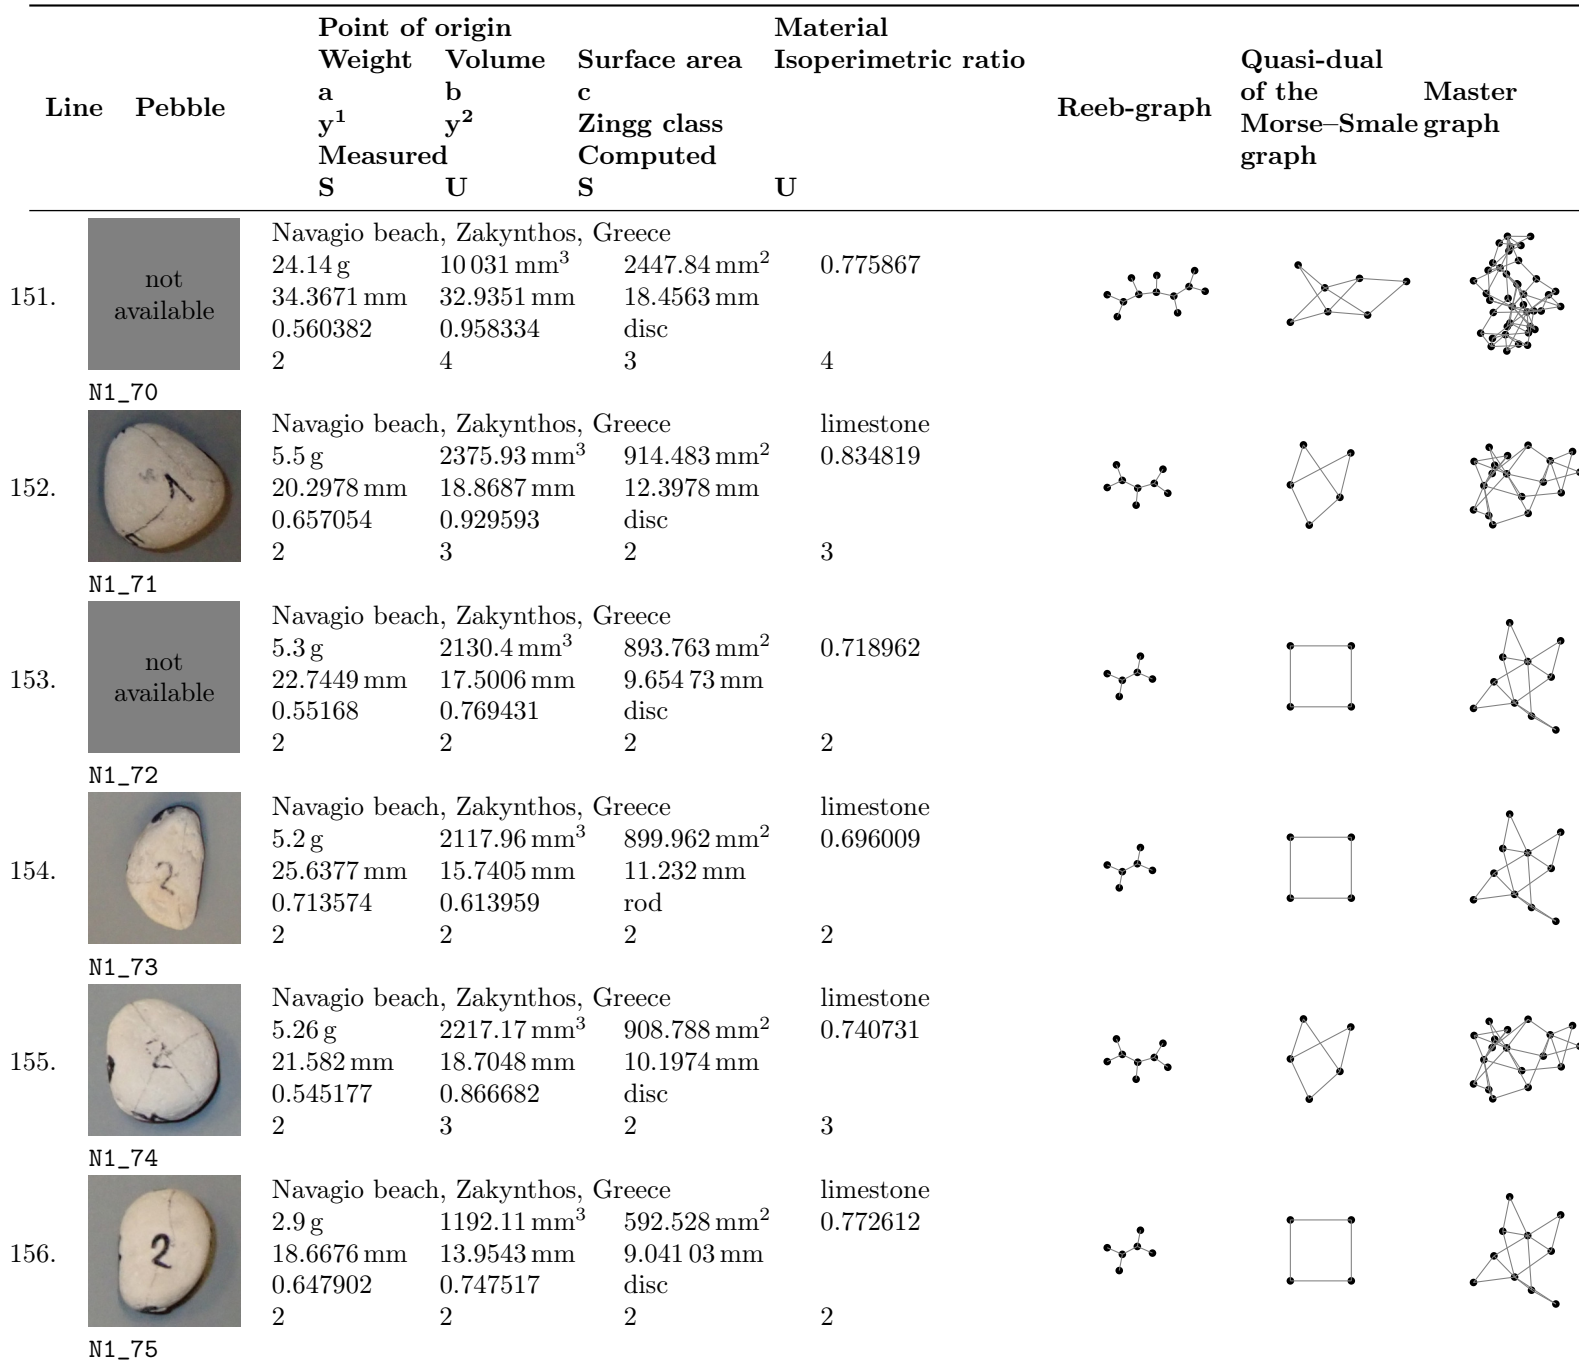 | Navagio beach, Zakynthos, Greece |                         |                         | limestone<br>0.740731 | 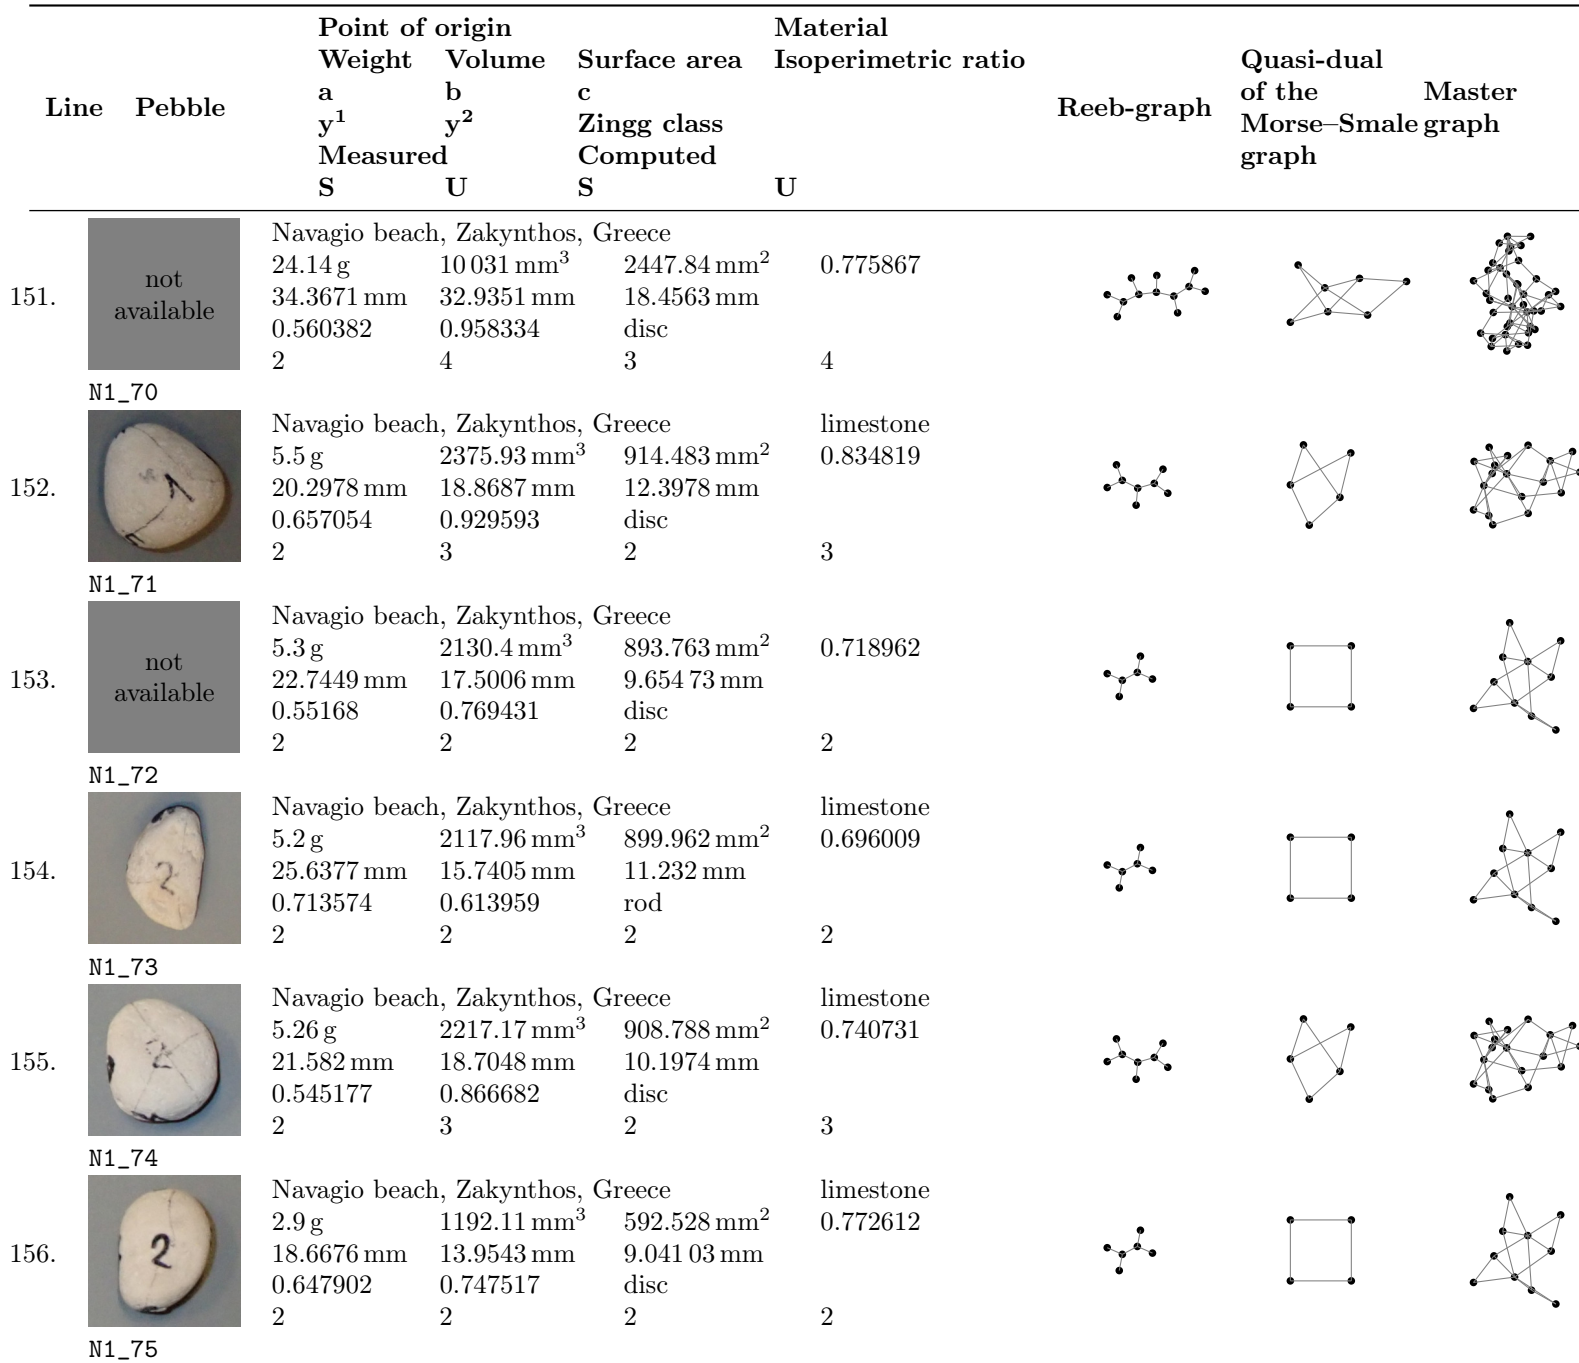 | 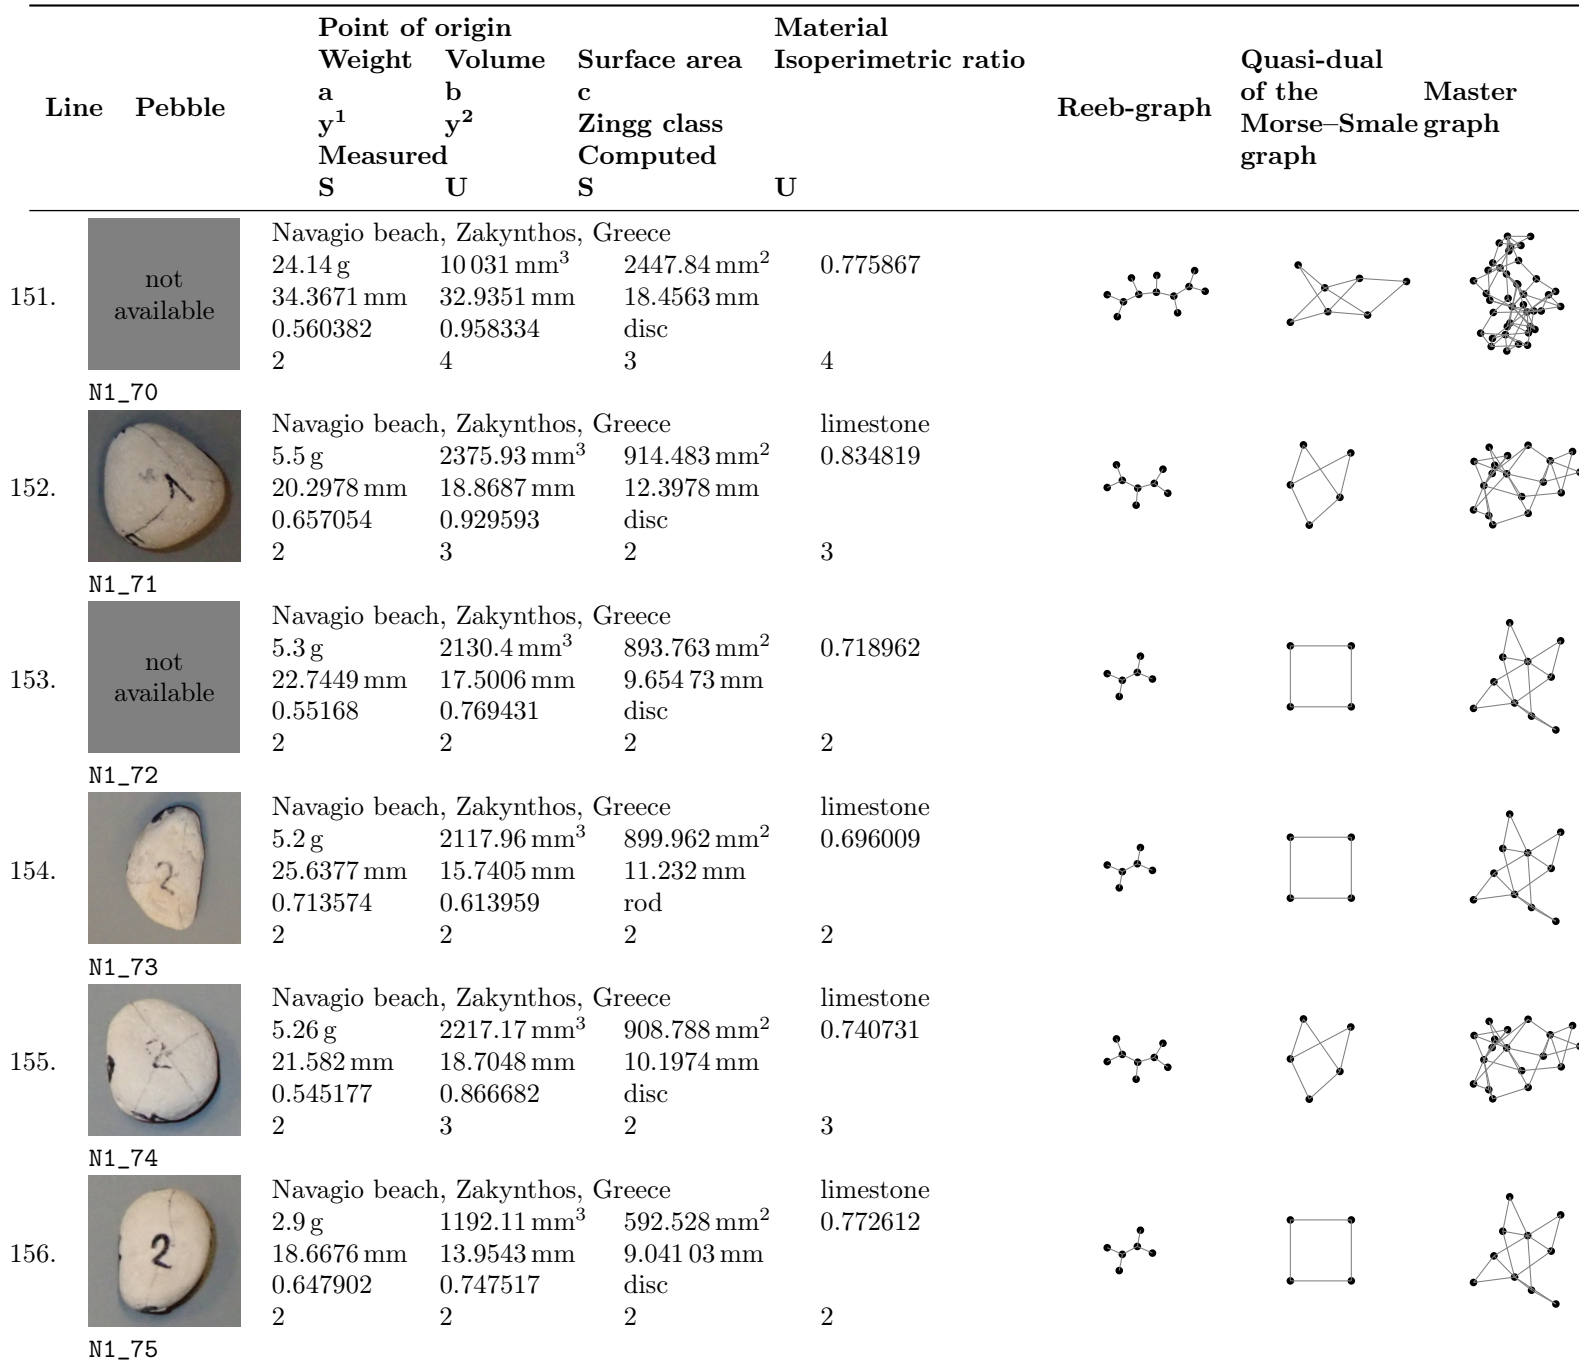 | 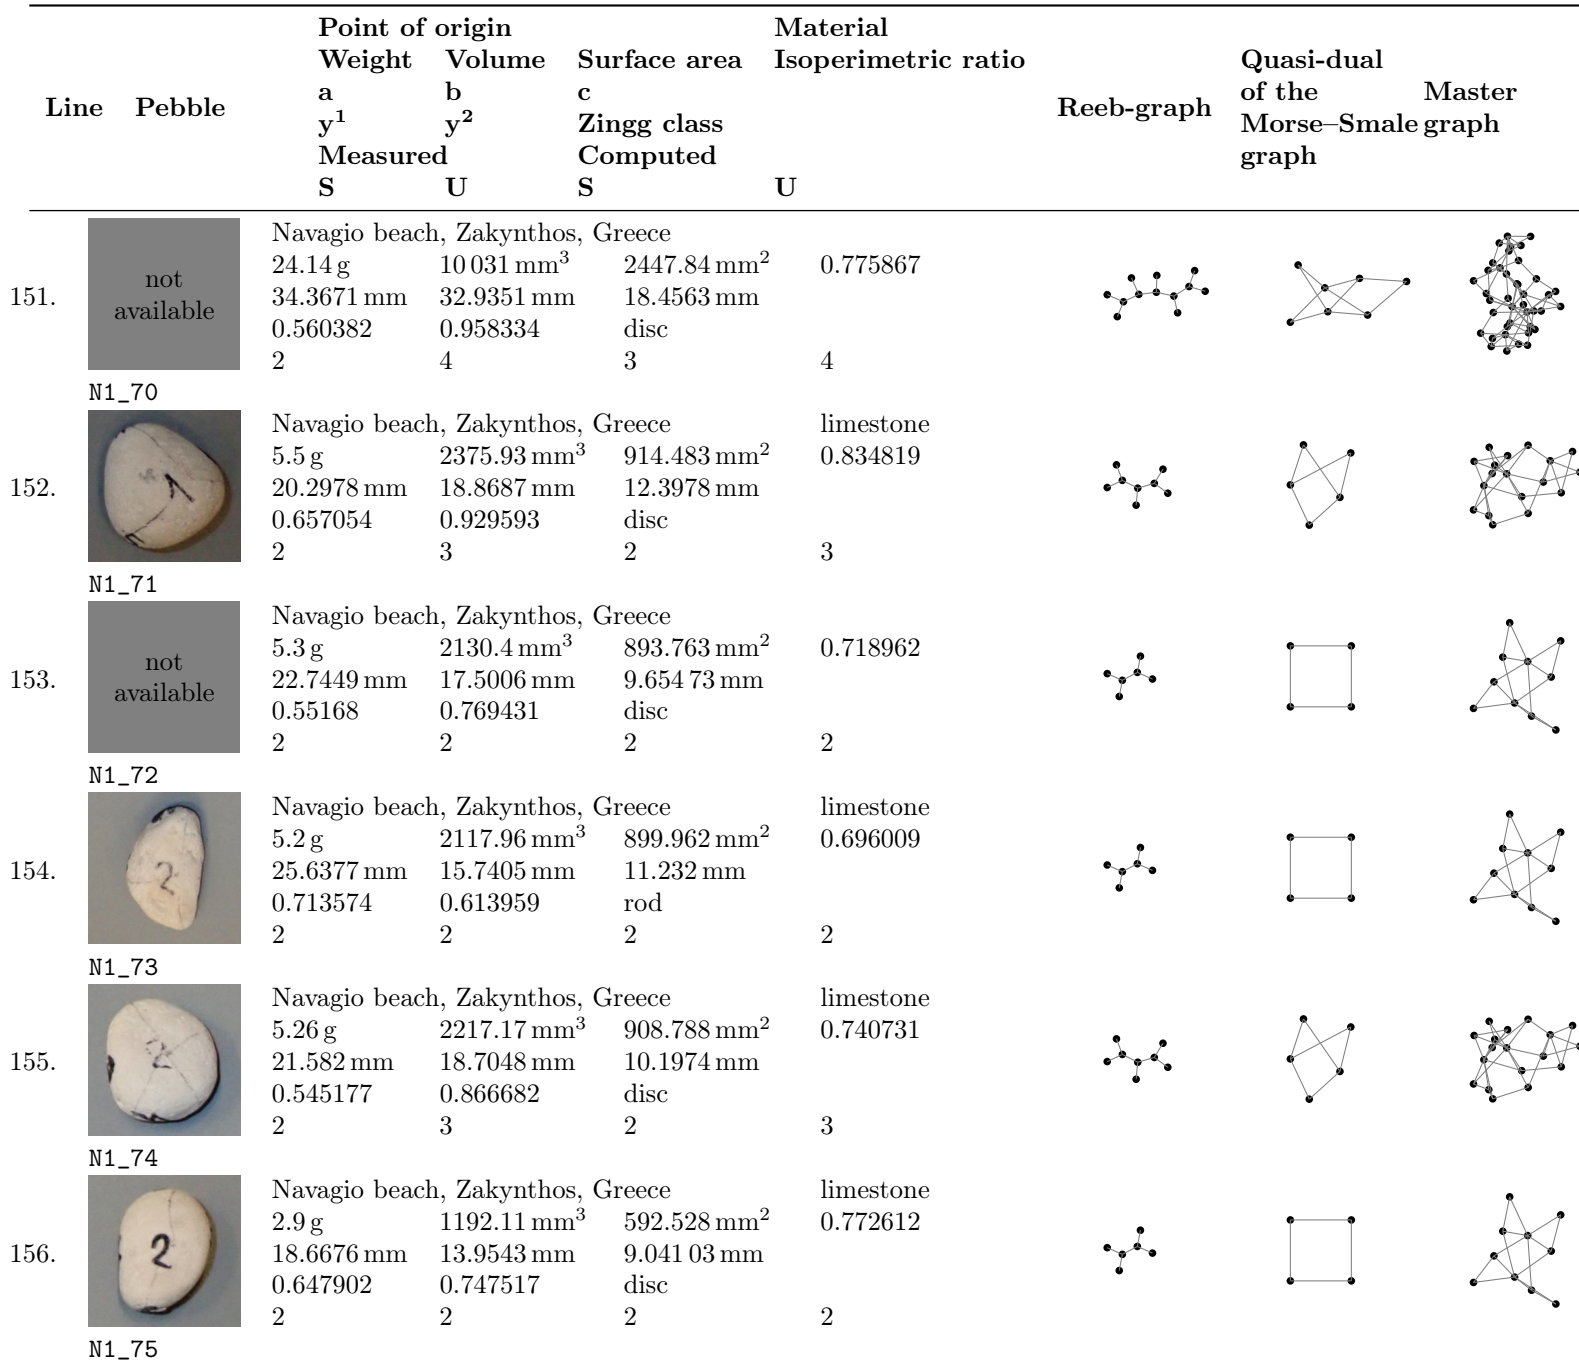 |
|      |                                                                                     | 5.26 g                           | 2217.17 mm <sup>3</sup> | 908.788 mm <sup>2</sup> |                       |                                                                                       |                                                                                       |                                                                                       |
|      |                                                                                     | 21.582 mm                        | 18.7048 mm              | 10.1974 mm              |                       |                                                                                       |                                                                                       |                                                                                       |
|      |                                                                                     | 0.545177                         | 0.866682                | disc                    |                       |                                                                                       |                                                                                       |                                                                                       |
|      |                                                                                     | 2                                | 3                       | 2                       |                       |                                                                                       |                                                                                       |                                                                                       |
|      | N1_74                                                                               |                                  |                         |                         |                       |                                                                                       |                                                                                       |                                                                                       |
| 156. | 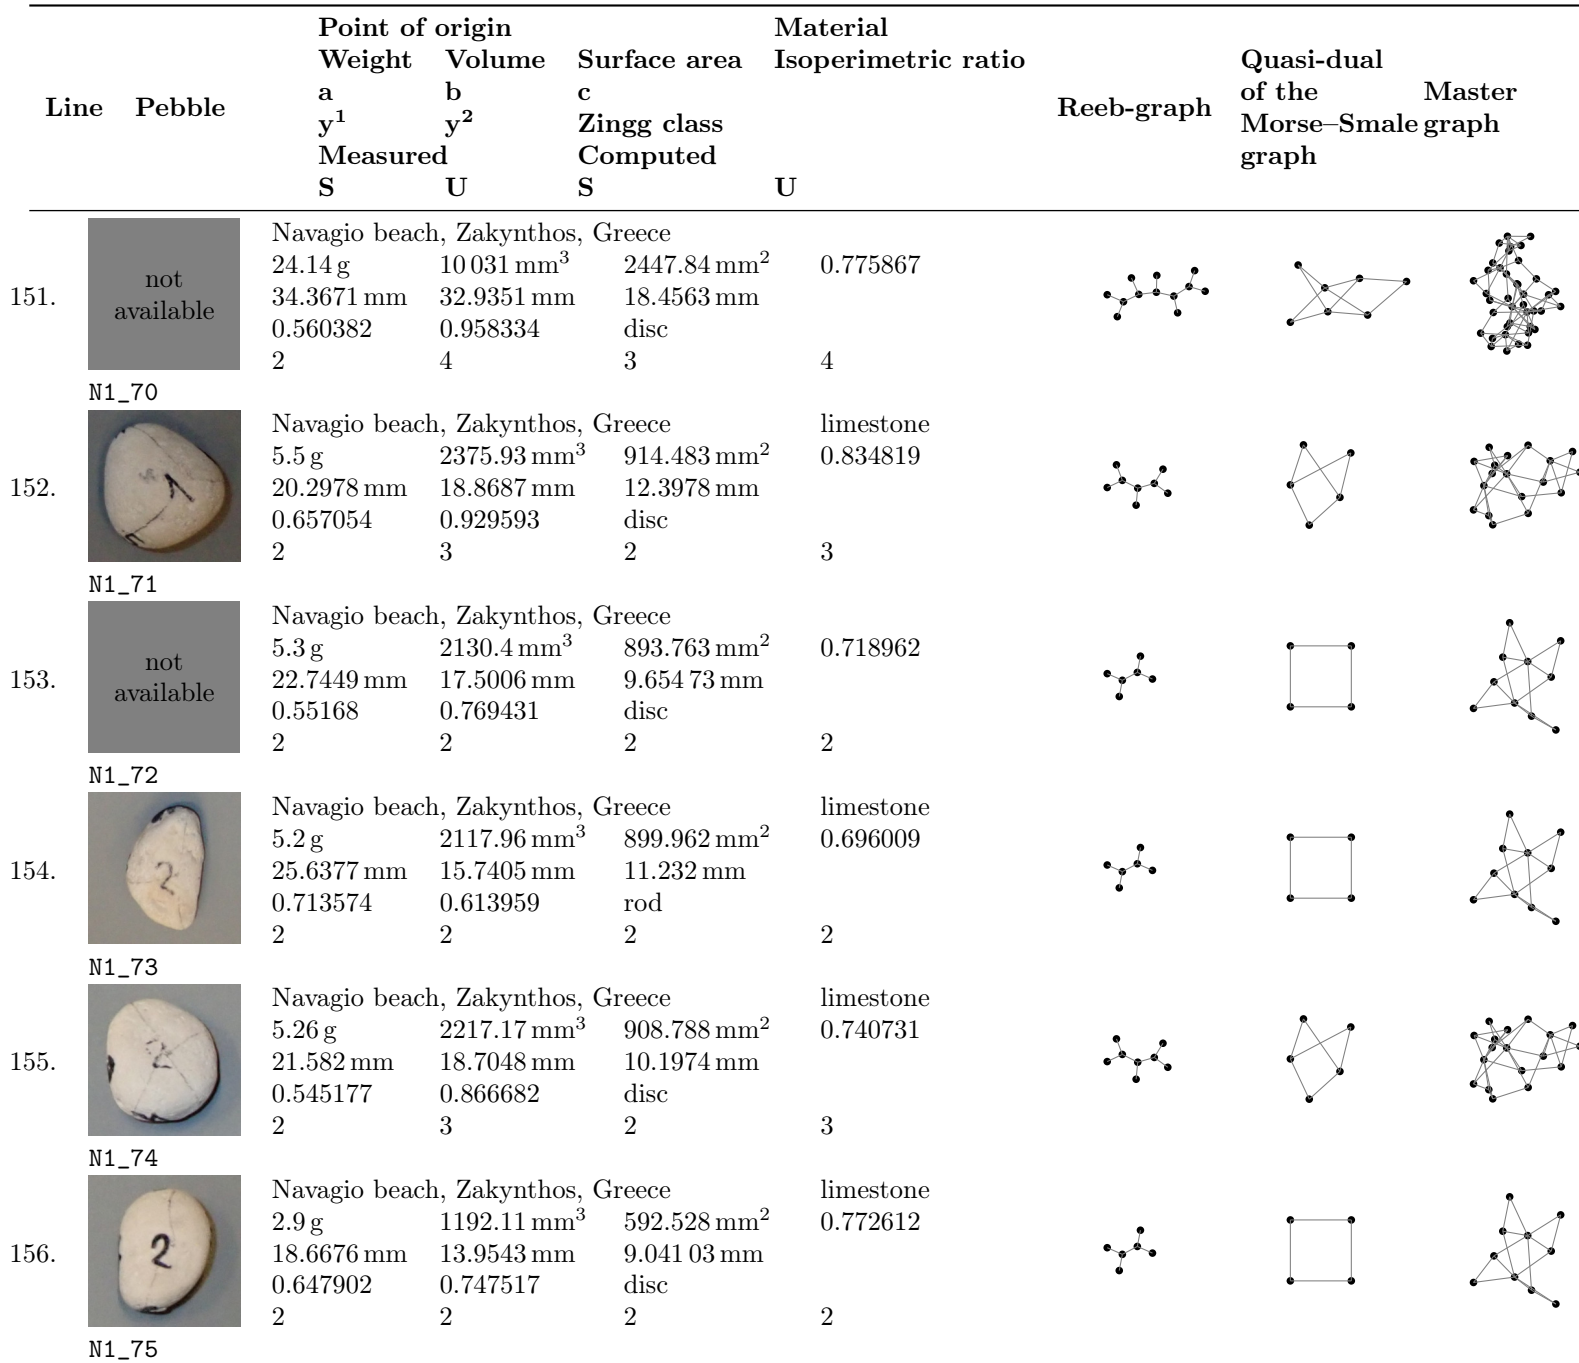 | Navagio beach, Zakynthos, Greece |                         |                         | limestone<br>0.772612 | 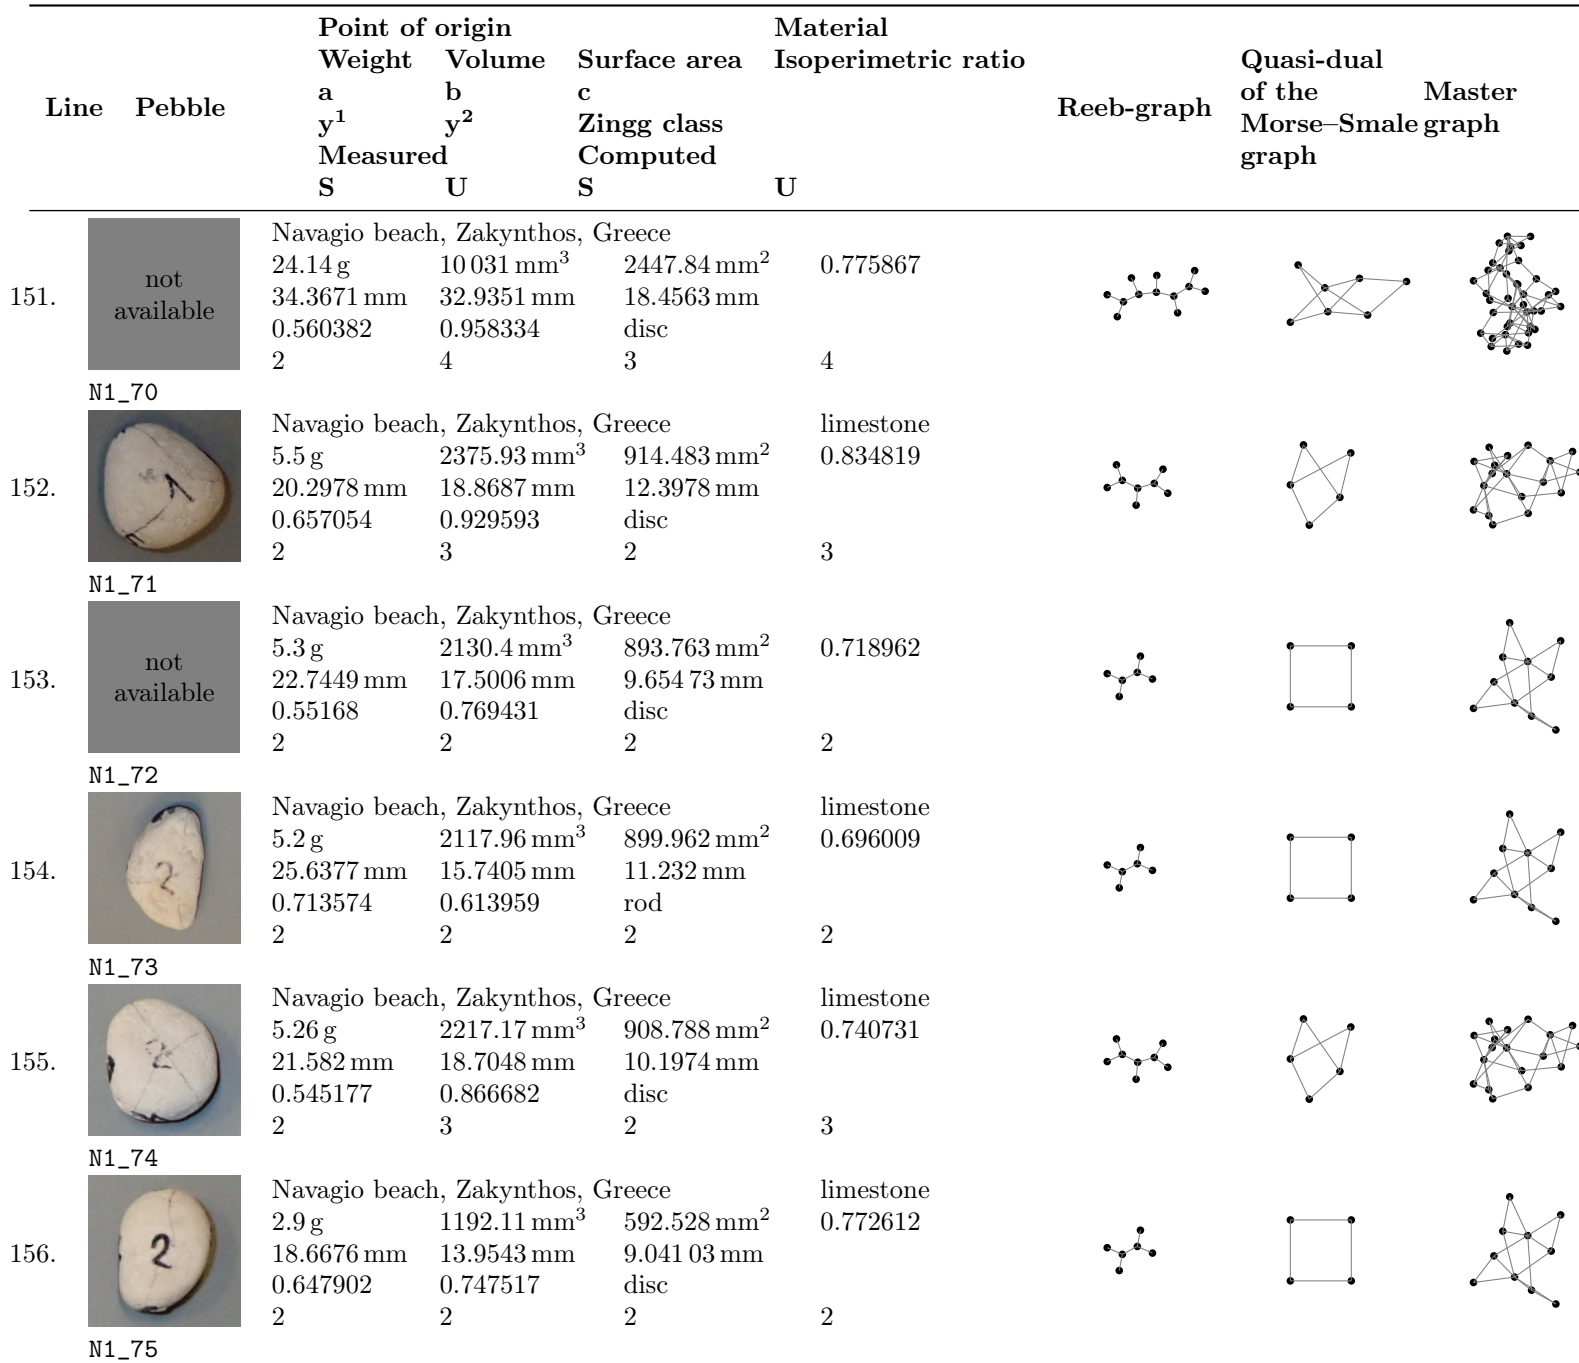 | 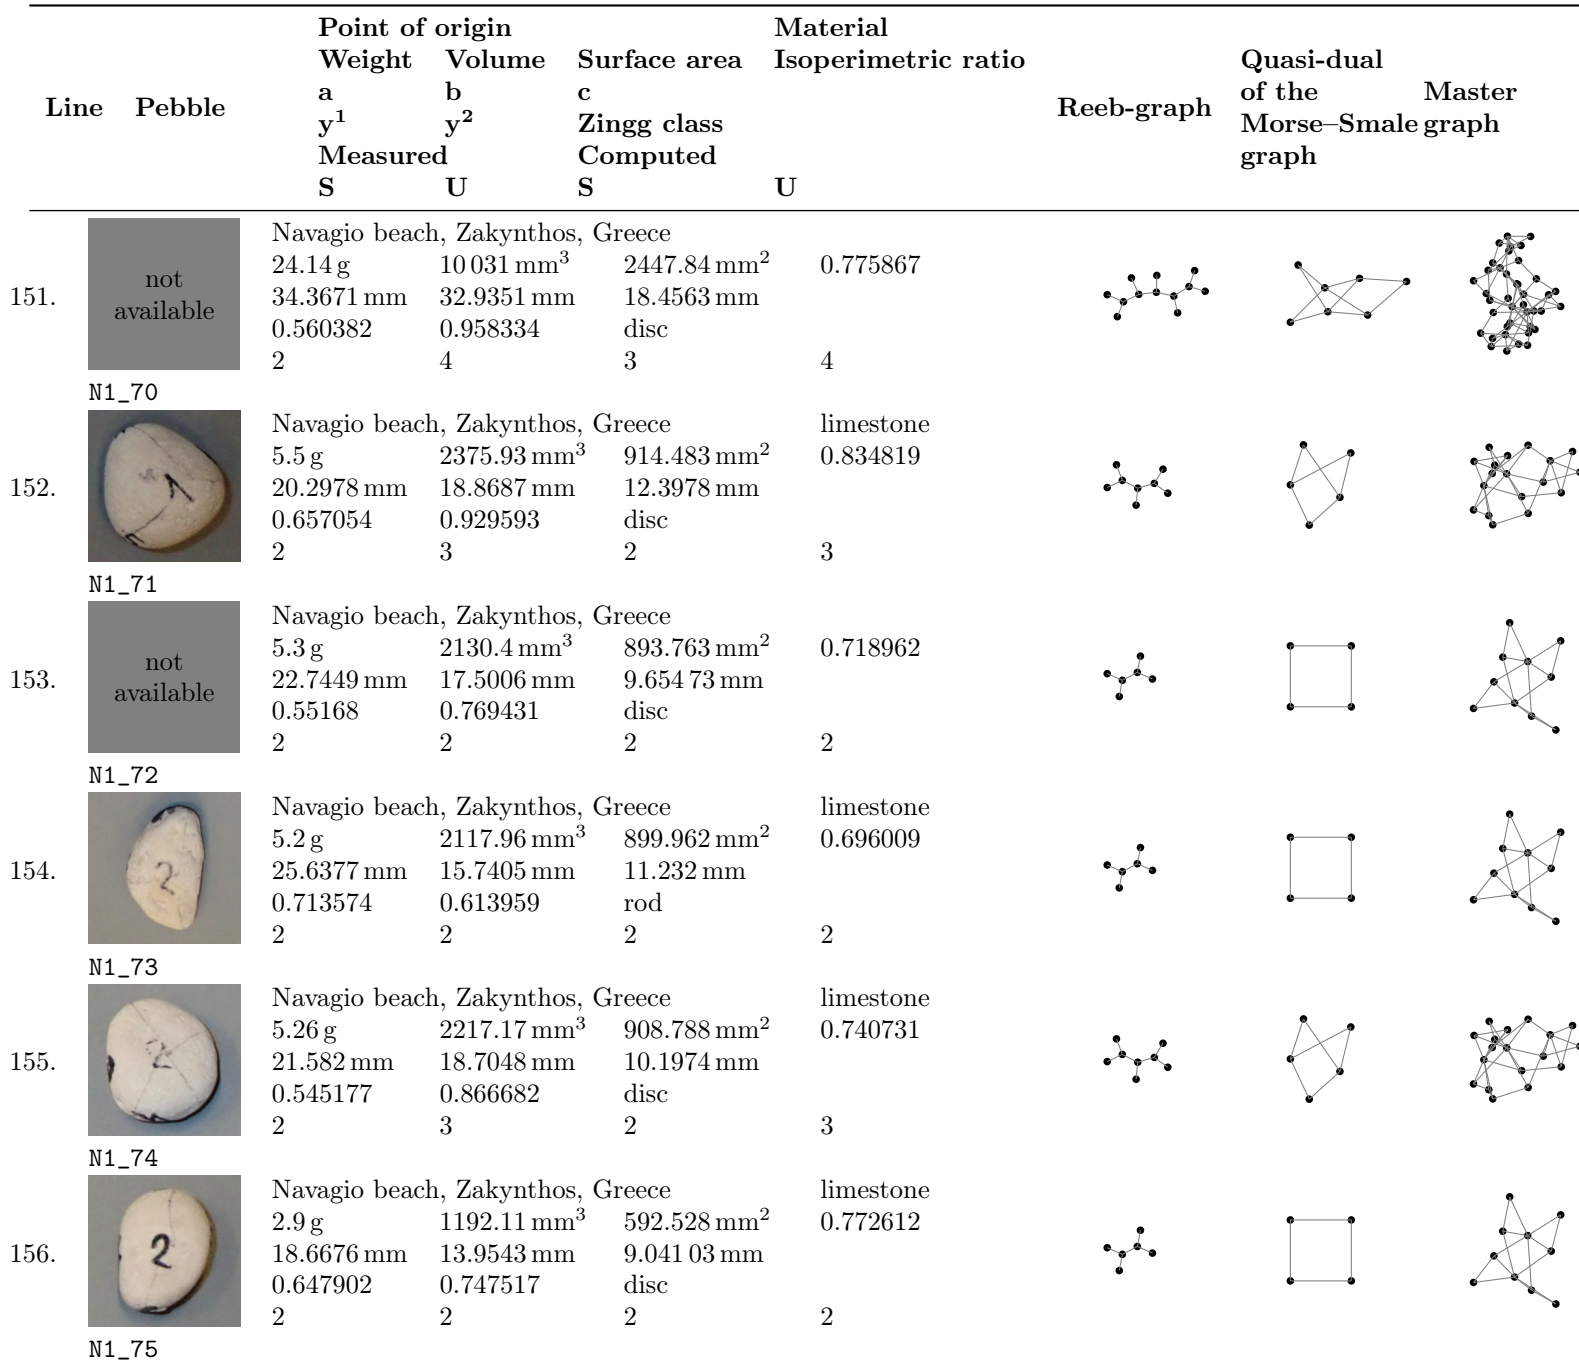 | 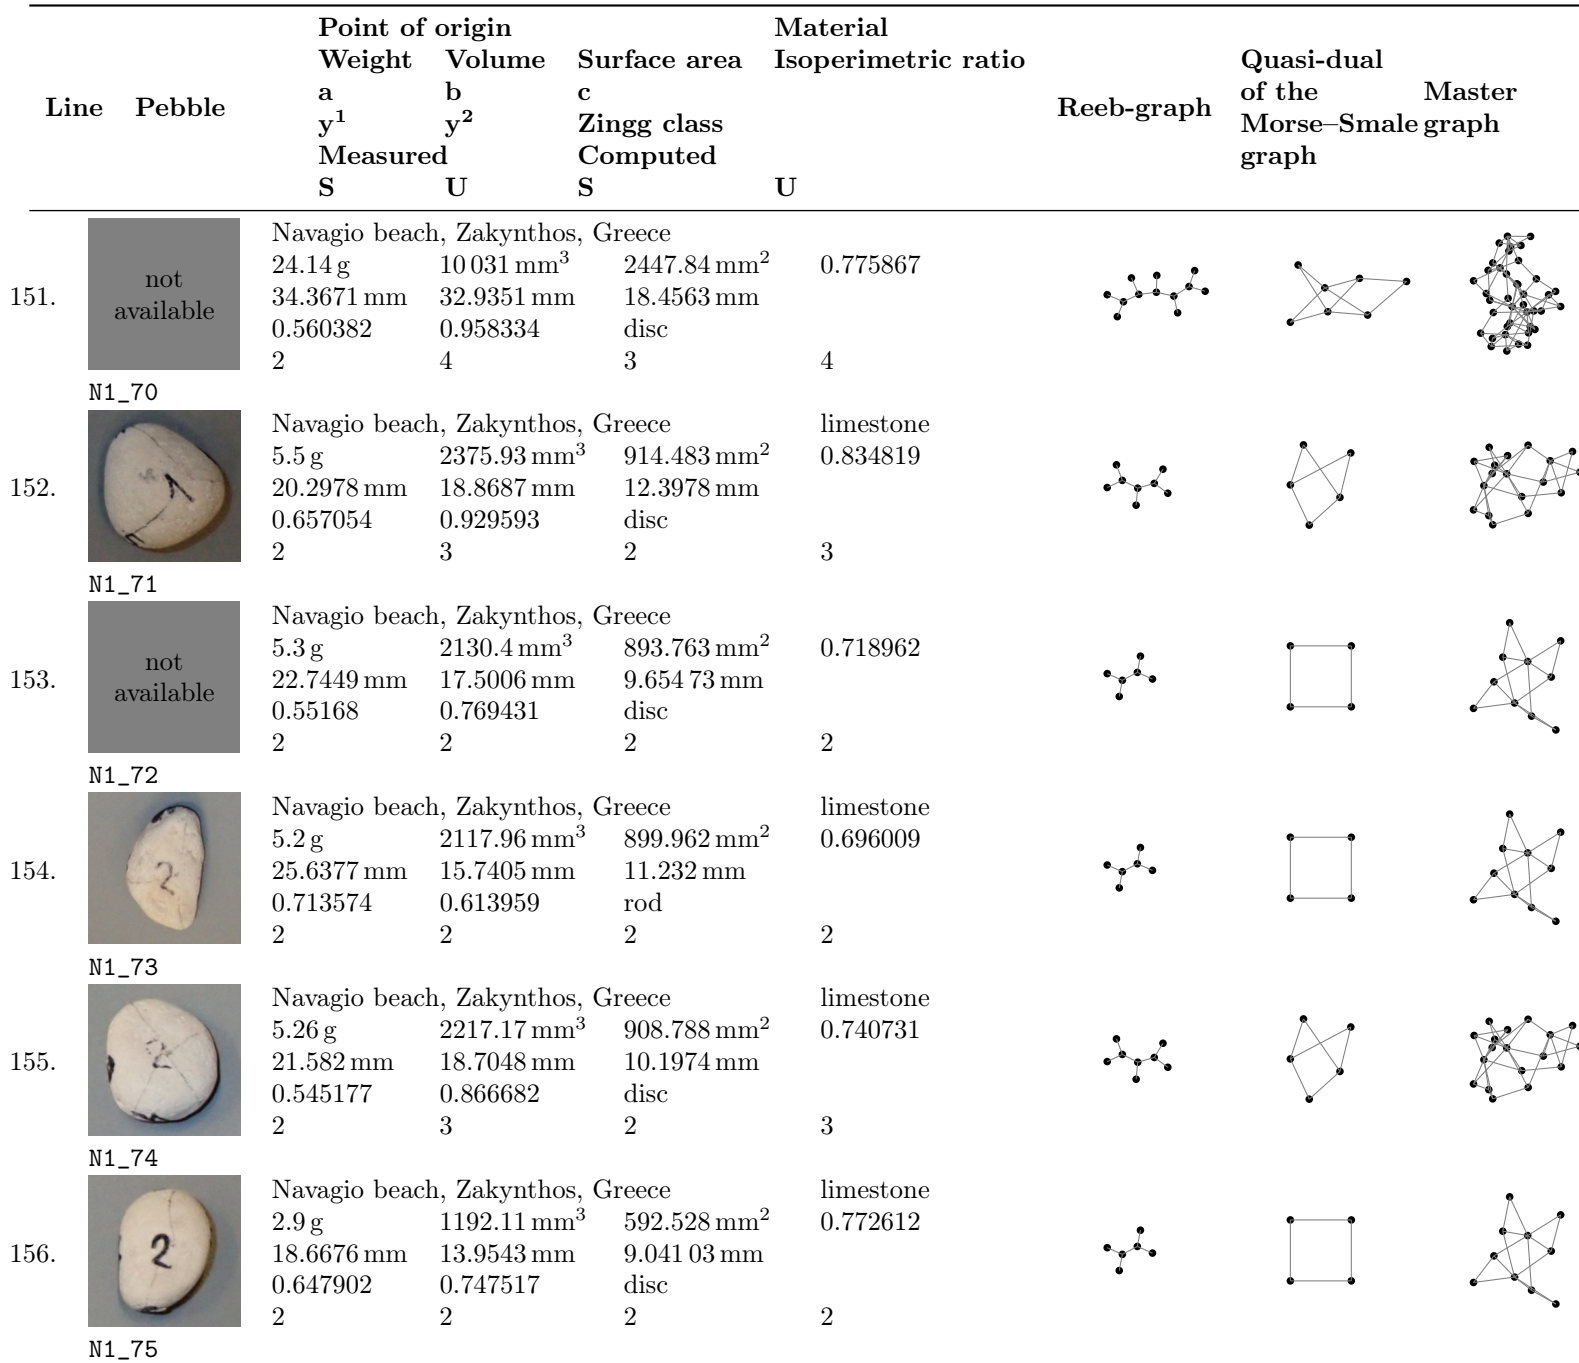 |
|      |                                                                                     | 2.9 g                            | 1192.11 mm <sup>3</sup> | 592.528 mm <sup>2</sup> |                       |                                                                                       |                                                                                       |                                                                                       |
|      |                                                                                     | 18.6676 mm                       | 13.9543 mm              | 9.041 03 mm             |                       |                                                                                       |                                                                                       |                                                                                       |
|      |                                                                                     | 0.647902                         | 0.747517                | disc                    |                       |                                                                                       |                                                                                       |                                                                                       |
|      |                                                                                     | 2                                | 2                       | 2                       |                       |                                                                                       |                                                                                       |                                                                                       |
|      | N1_75                                                                               |                                  |                         |                         |                       |                                                                                       |                                                                                       |                                                                                       |

| Line | Pebble                                                                              | Point of origin                                                           |                                                        |                                                     | Material                       | Isoperimetric ratio | Reeb-graph                                                                            | Quasi-dual<br>of the<br>Morse–Smale<br>graph                                          | Master                                                                                |
|------|-------------------------------------------------------------------------------------|---------------------------------------------------------------------------|--------------------------------------------------------|-----------------------------------------------------|--------------------------------|---------------------|---------------------------------------------------------------------------------------|---------------------------------------------------------------------------------------|---------------------------------------------------------------------------------------|
|      |                                                                                     | Weight                                                                    | Volume                                                 | Surface area                                        |                                |                     |                                                                                       |                                                                                       |                                                                                       |
|      |                                                                                     | a                                                                         | b                                                      | c                                                   |                                |                     |                                                                                       |                                                                                       |                                                                                       |
|      |                                                                                     | y <sup>1</sup><br>Measured<br>S                                           | y <sup>2</sup><br>U                                    | Zingg class<br>Computed<br>S                        |                                |                     |                                                                                       |                                                                                       |                                                                                       |
| 157. | 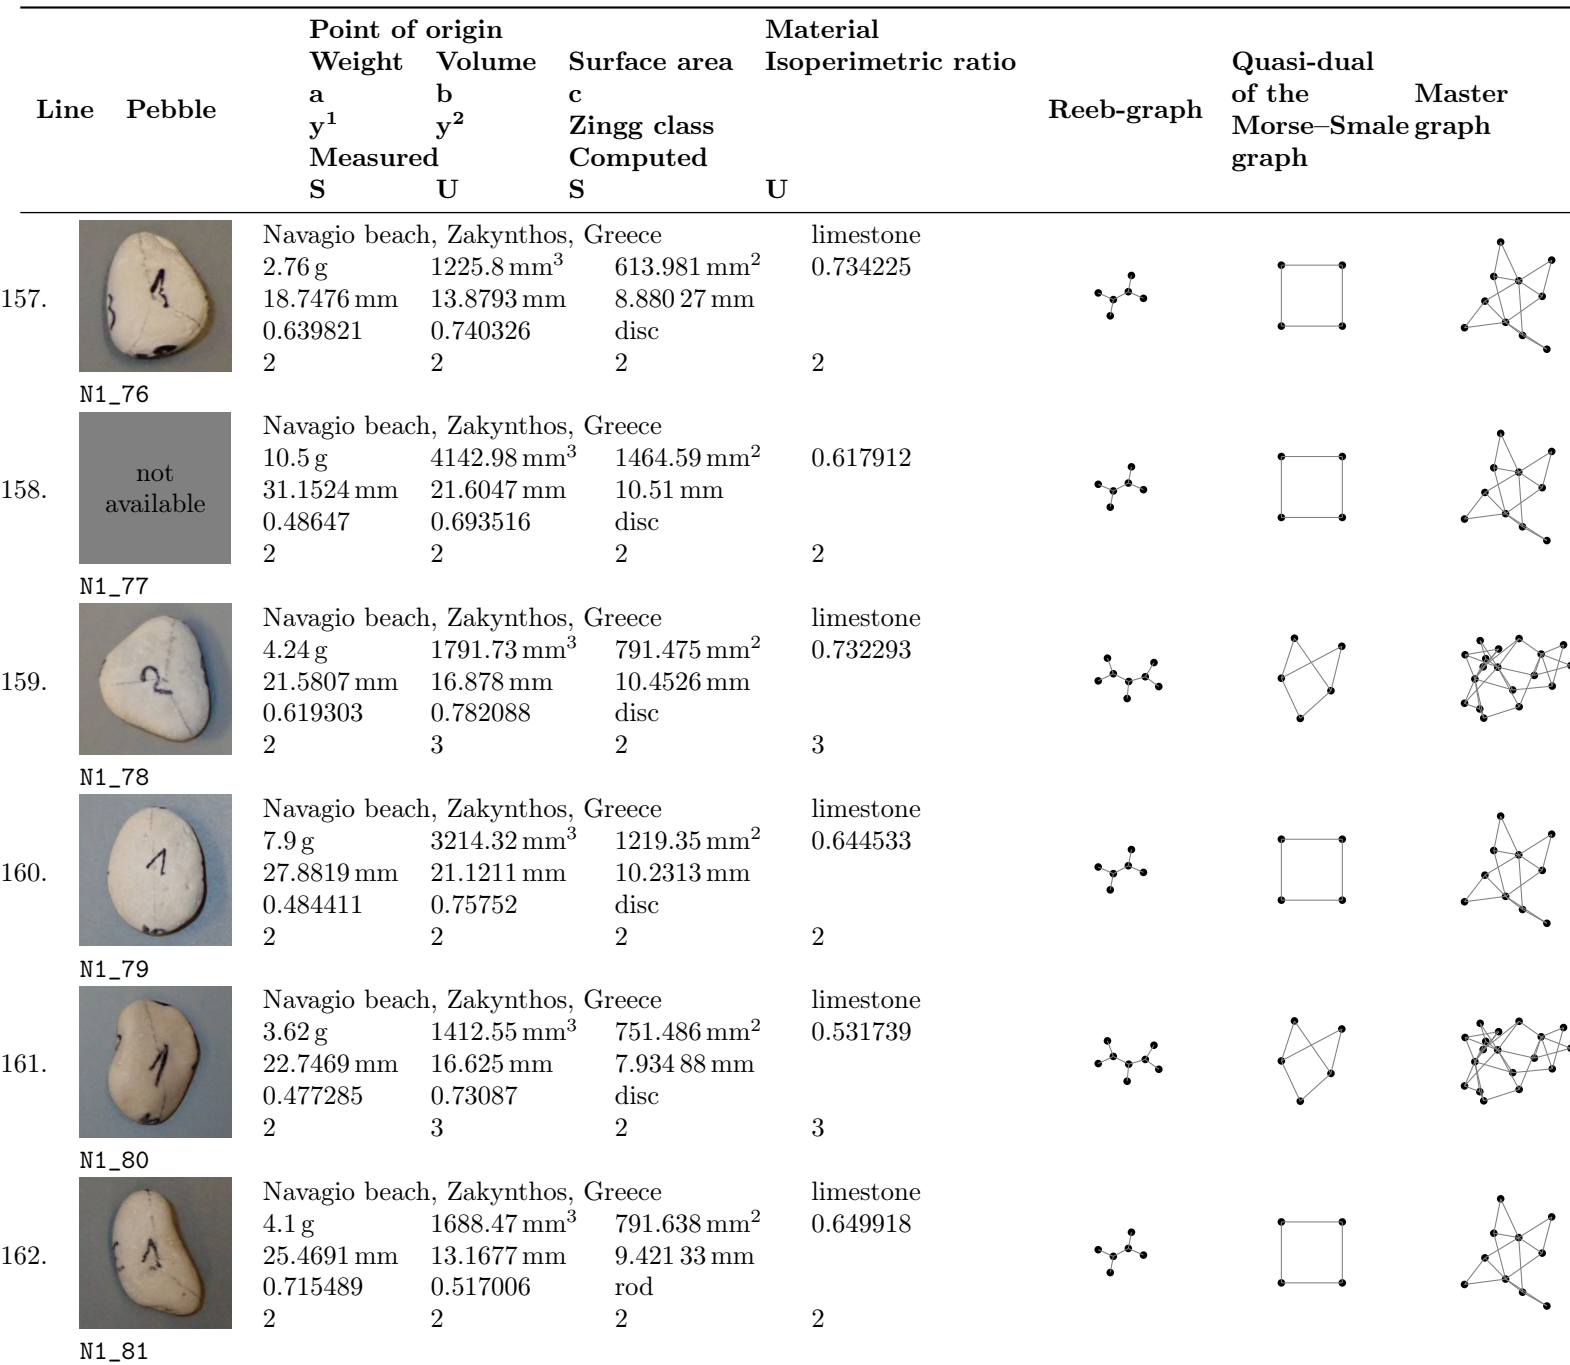   | Navagio beach, Zakynthos, Greece<br>2.76 g<br>18.7476 mm<br>0.639821<br>2 | 1225.8 mm <sup>3</sup><br>13.8793 mm<br>0.740326<br>2  | 613.981 mm <sup>2</sup><br>8.880 27 mm<br>disc<br>2 | limestone<br>0.734225<br><br>2 |                     | 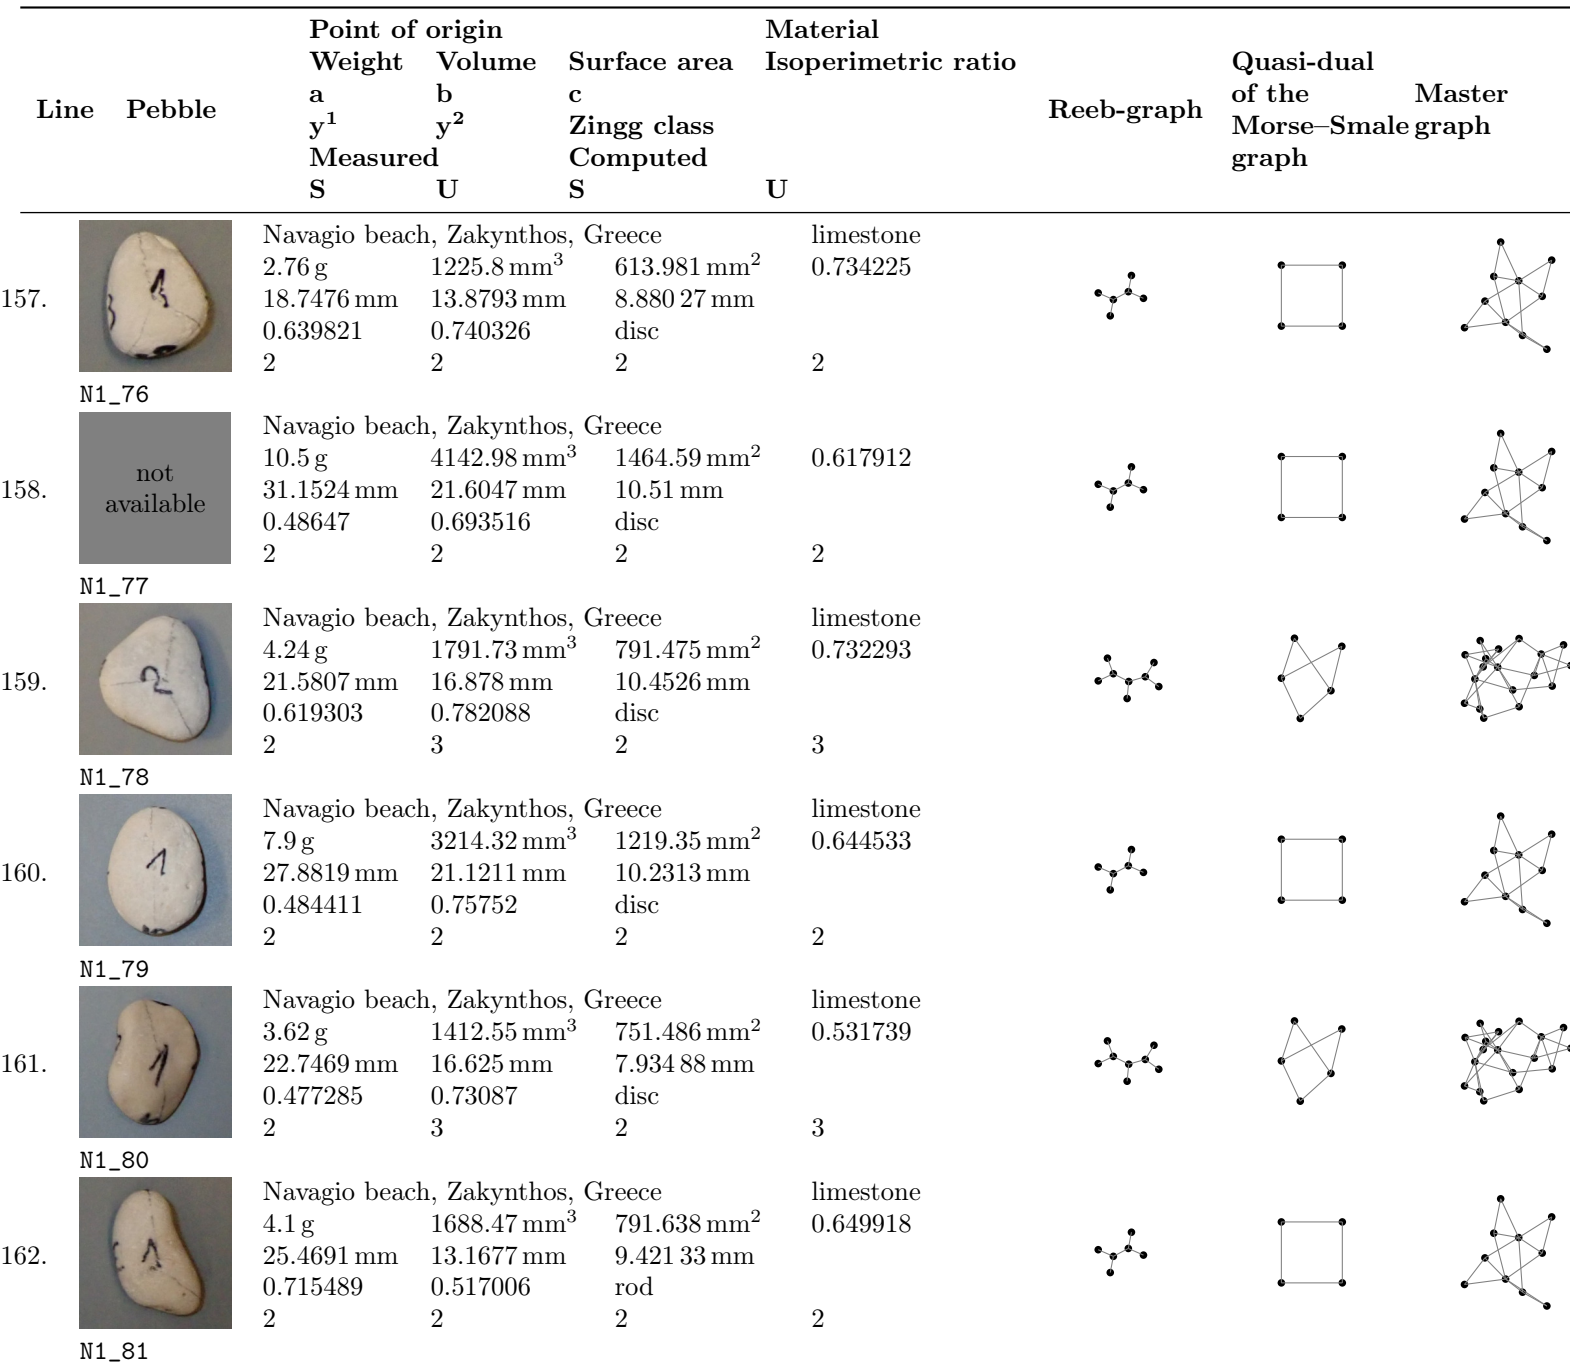   | 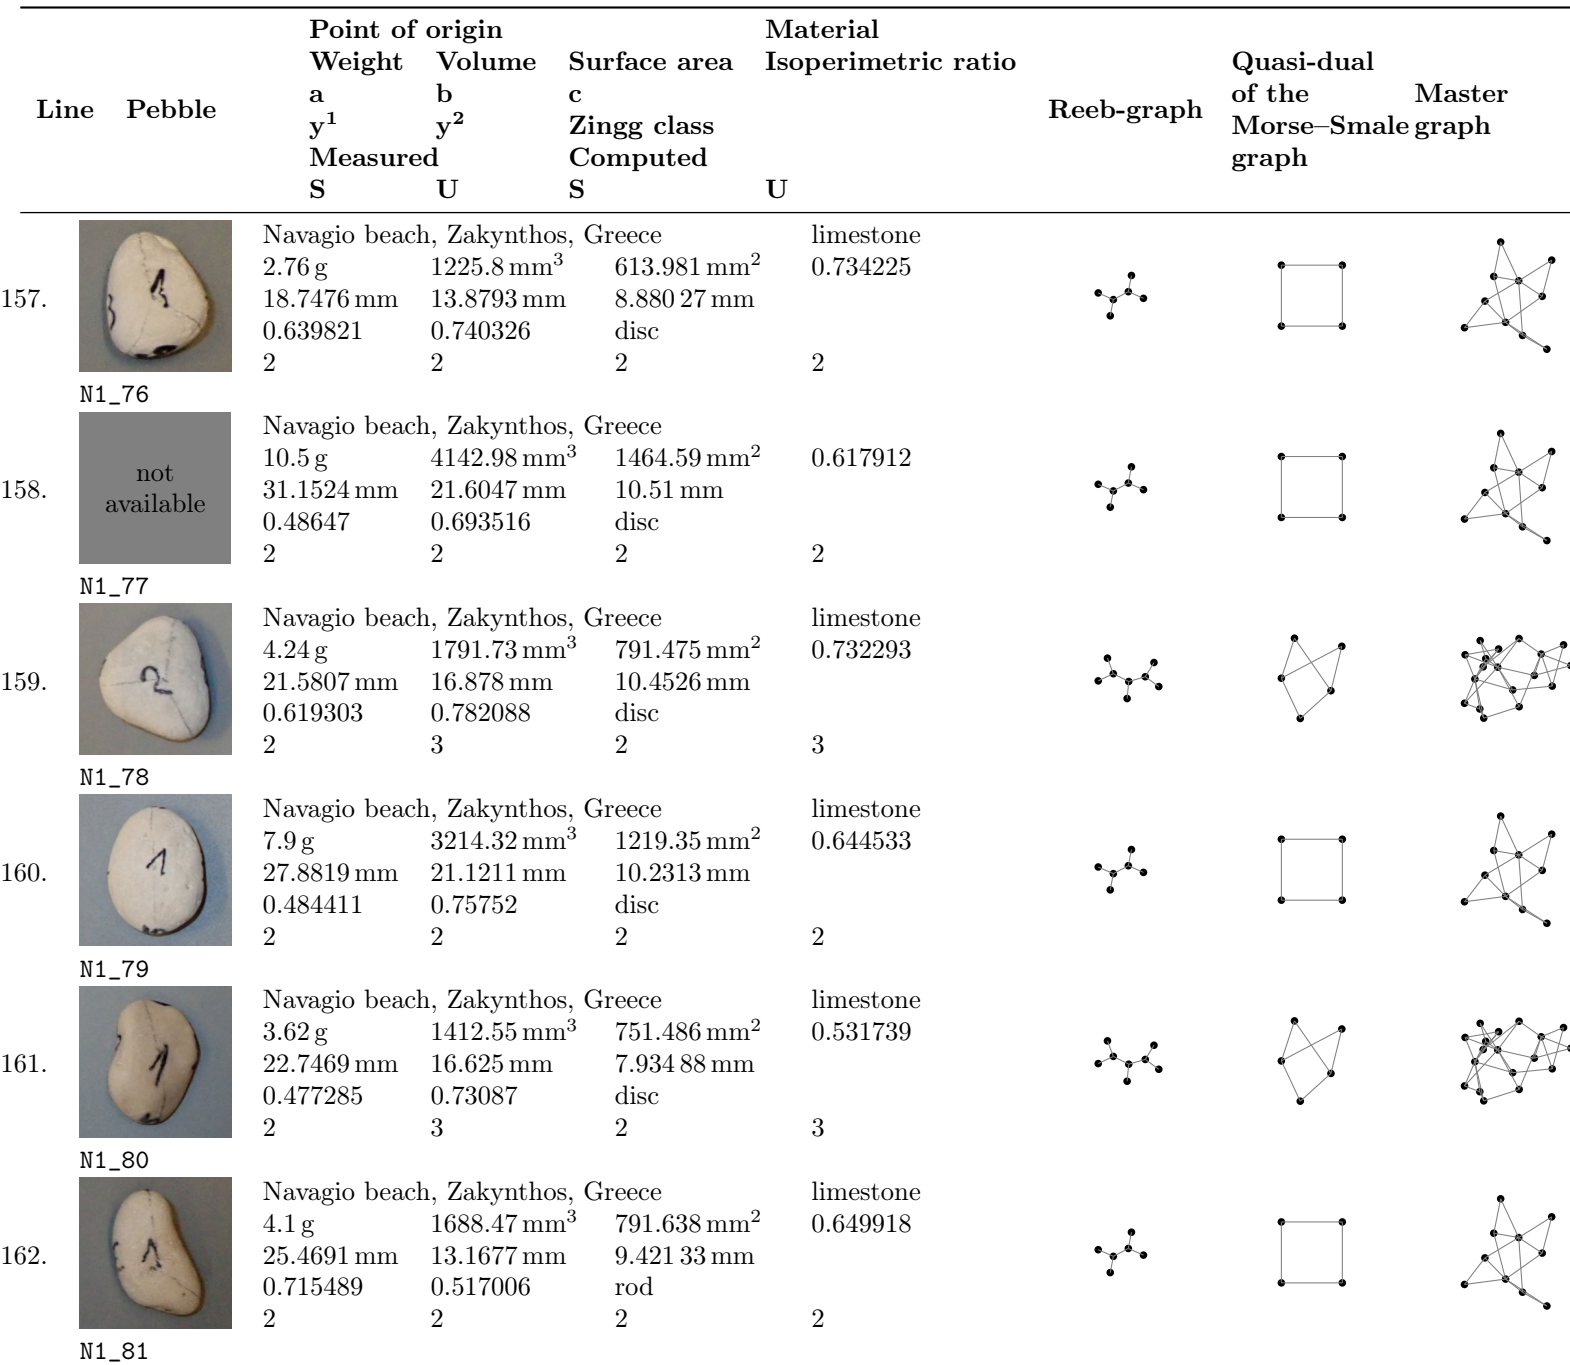   | 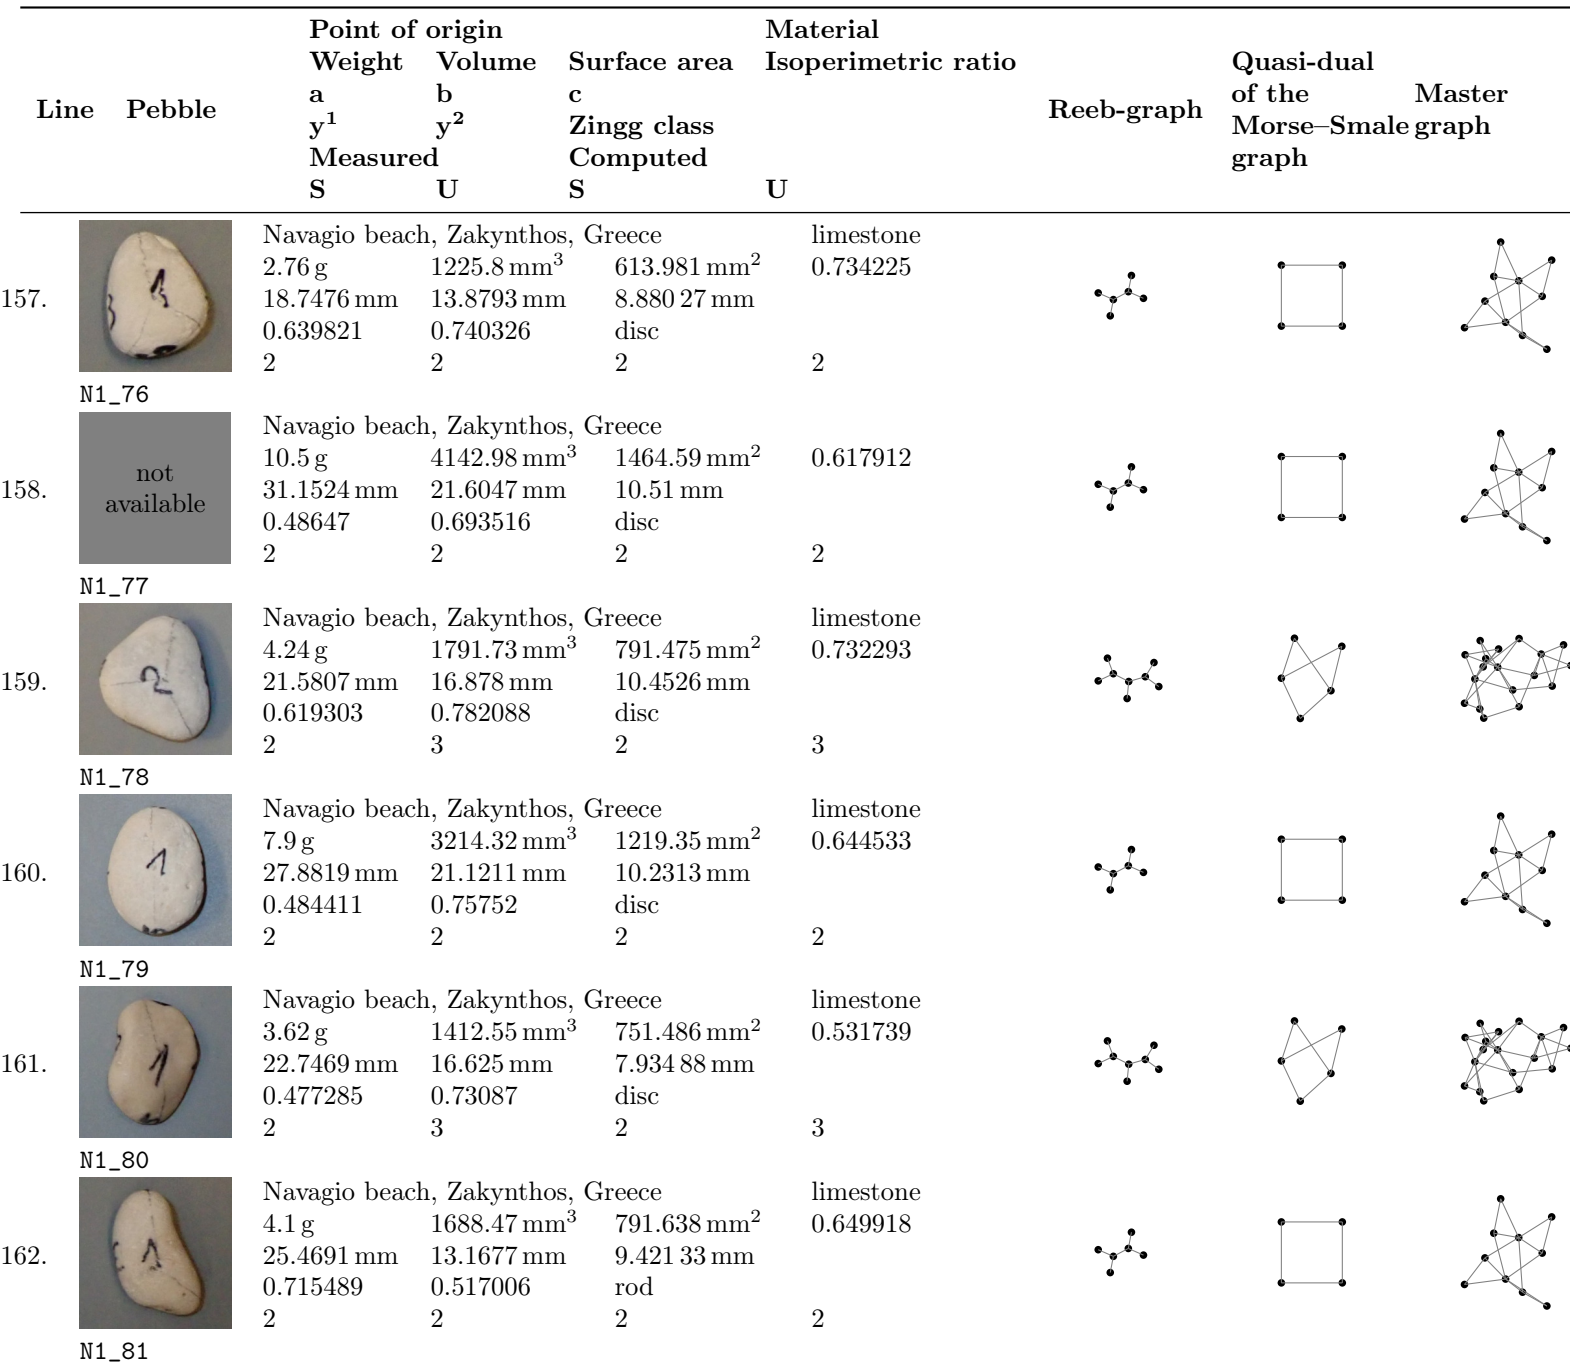   |
|      | N1_76                                                                               |                                                                           |                                                        |                                                     |                                |                     |                                                                                       |                                                                                       |                                                                                       |
| 158. | 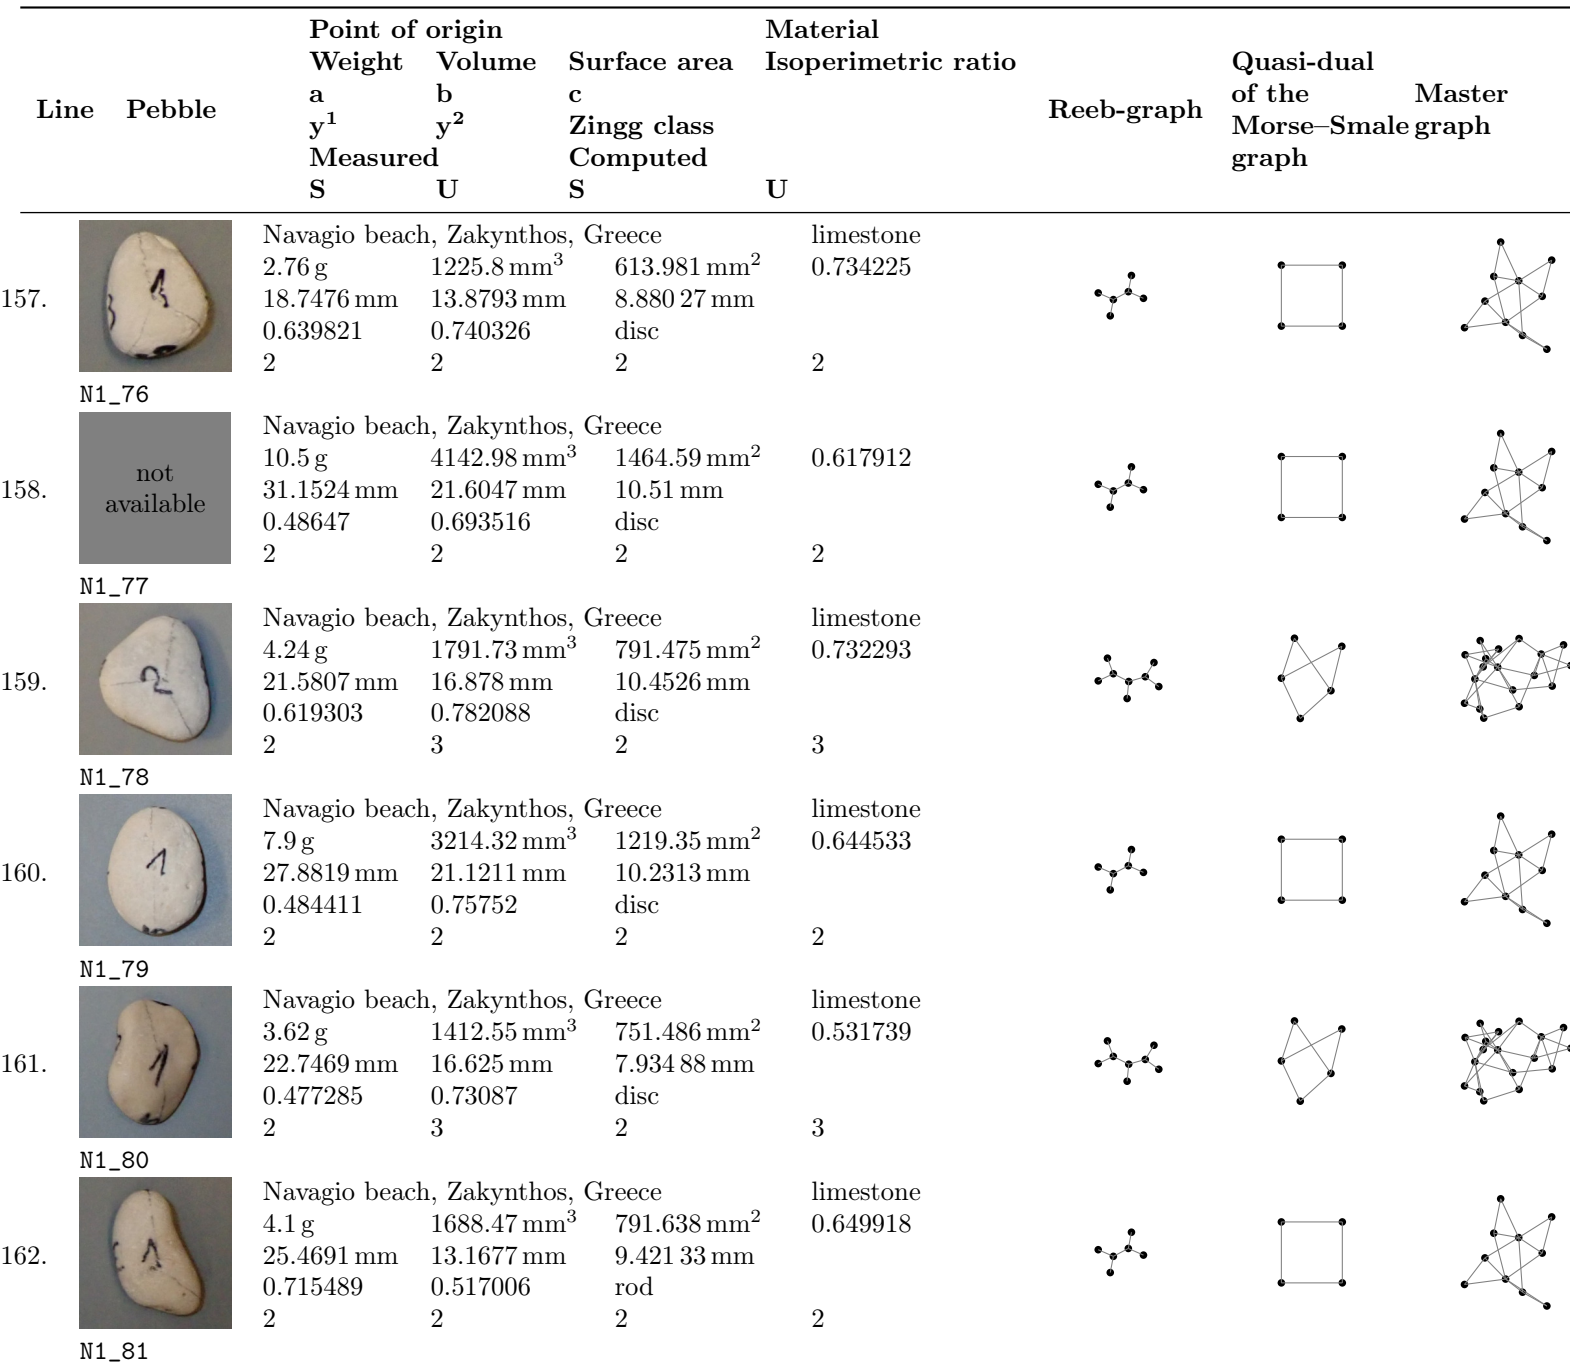   | Navagio beach, Zakynthos, Greece<br>10.5 g<br>31.1524 mm<br>0.48647<br>2  | 4142.98 mm <sup>3</sup><br>21.6047 mm<br>0.693516<br>2 | 1464.59 mm <sup>2</sup><br>10.51 mm<br>disc<br>2    | 0.617912<br><br>2              |                     | 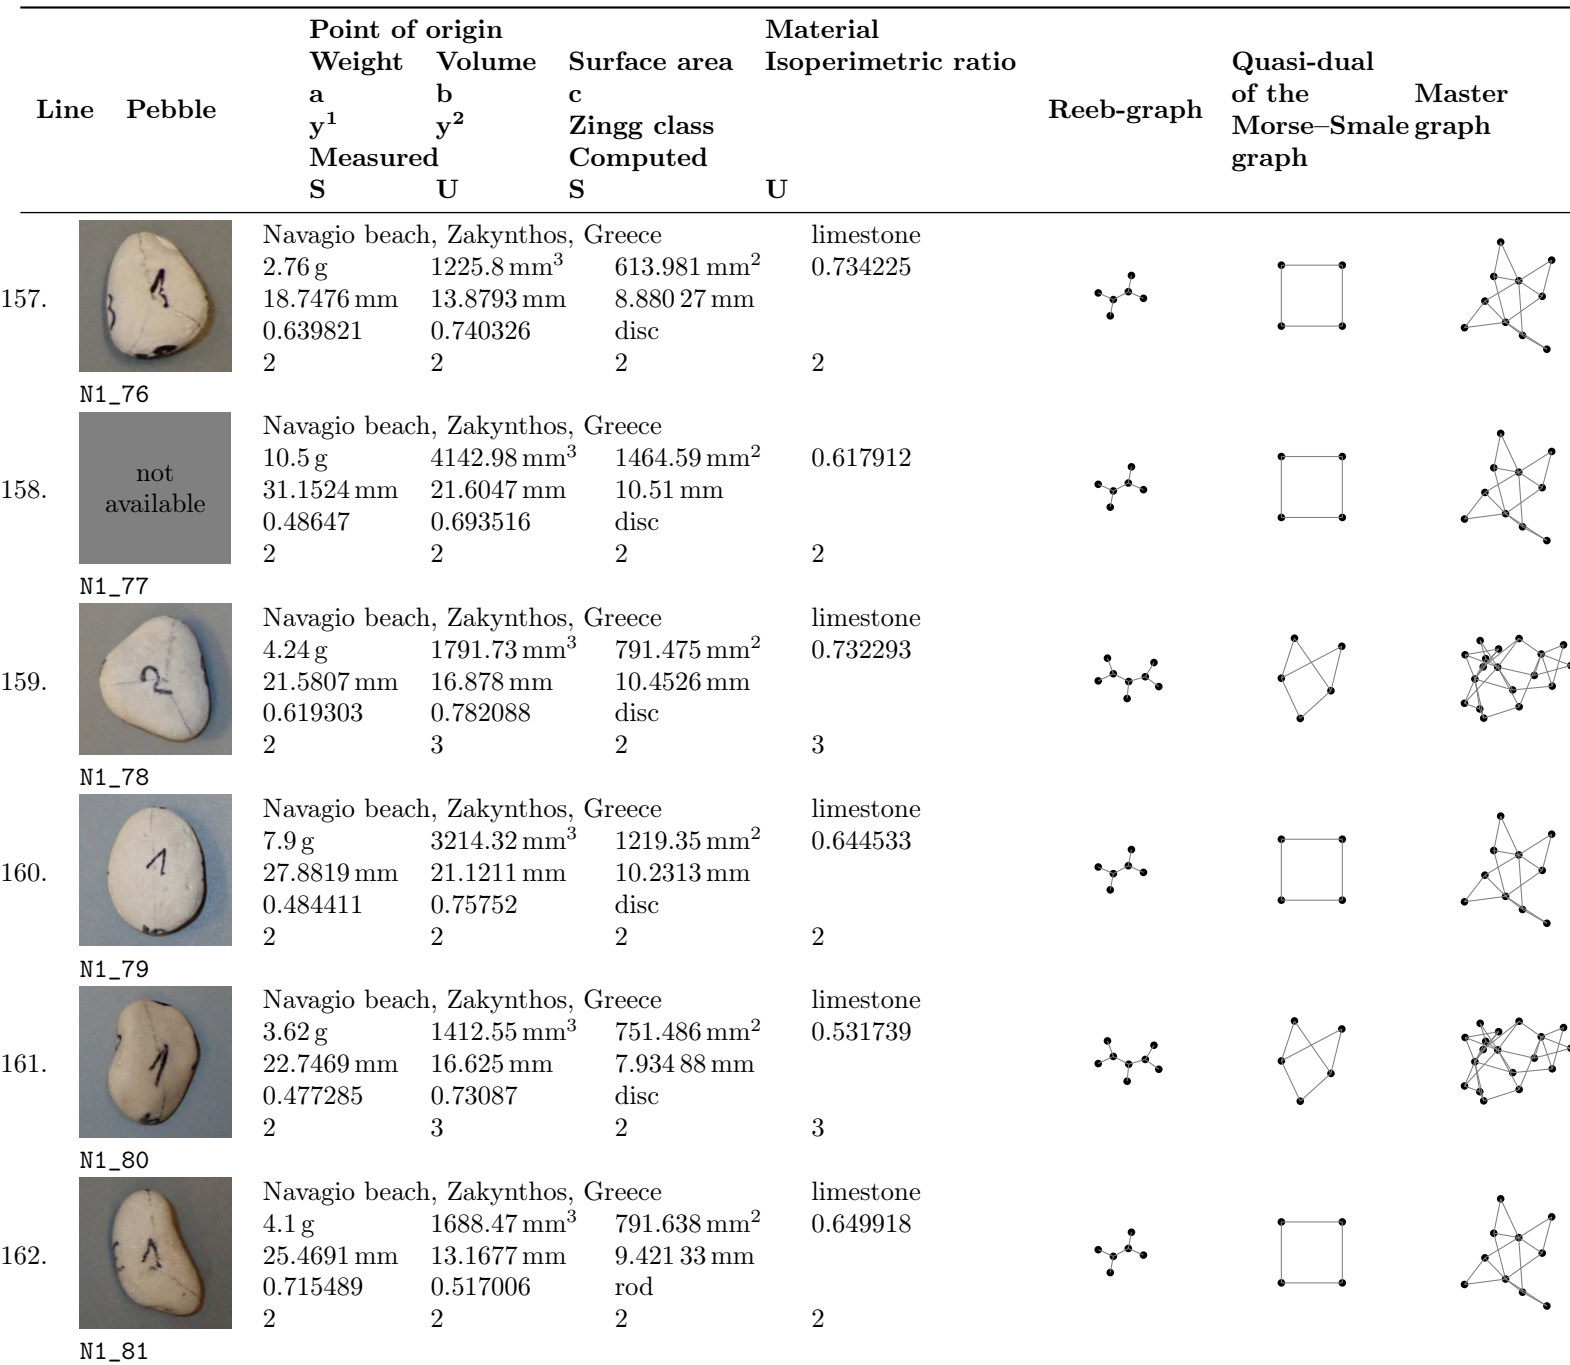   | 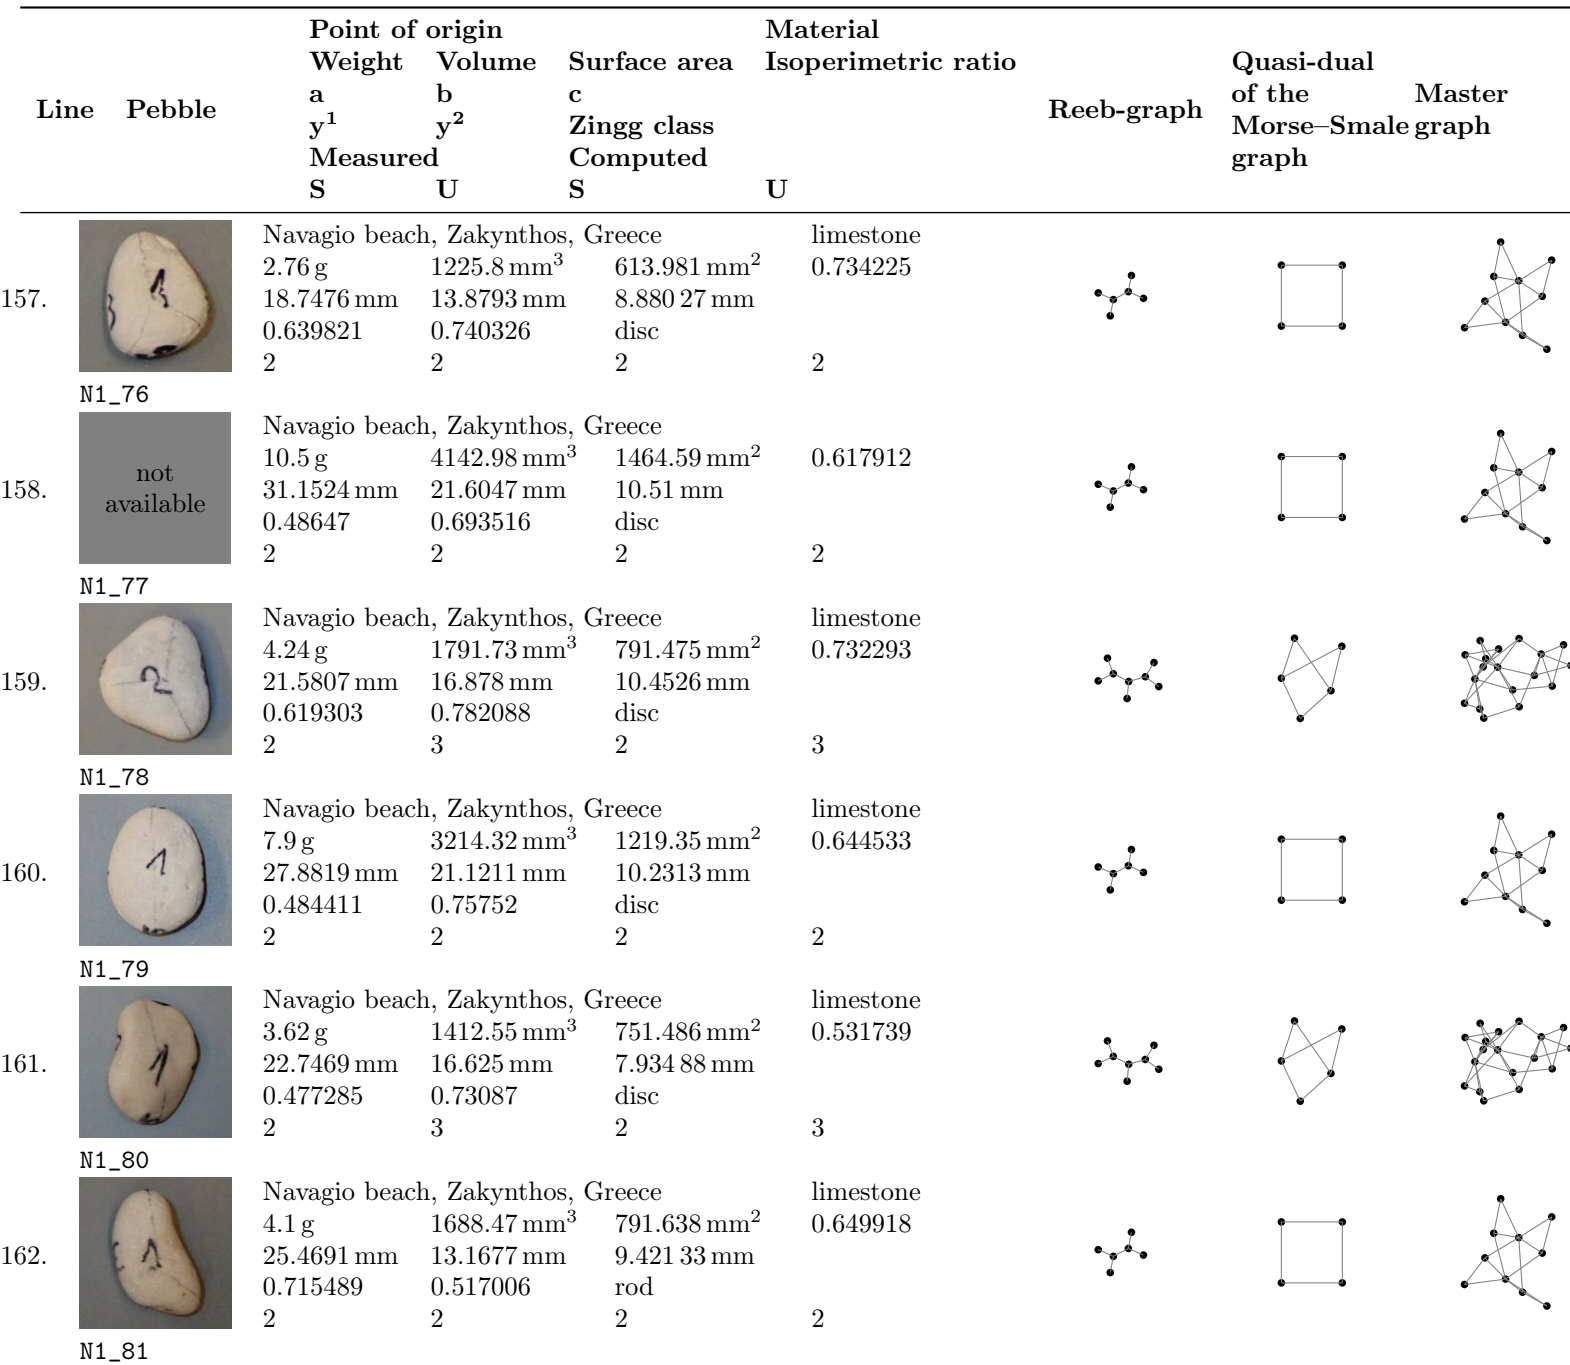   | 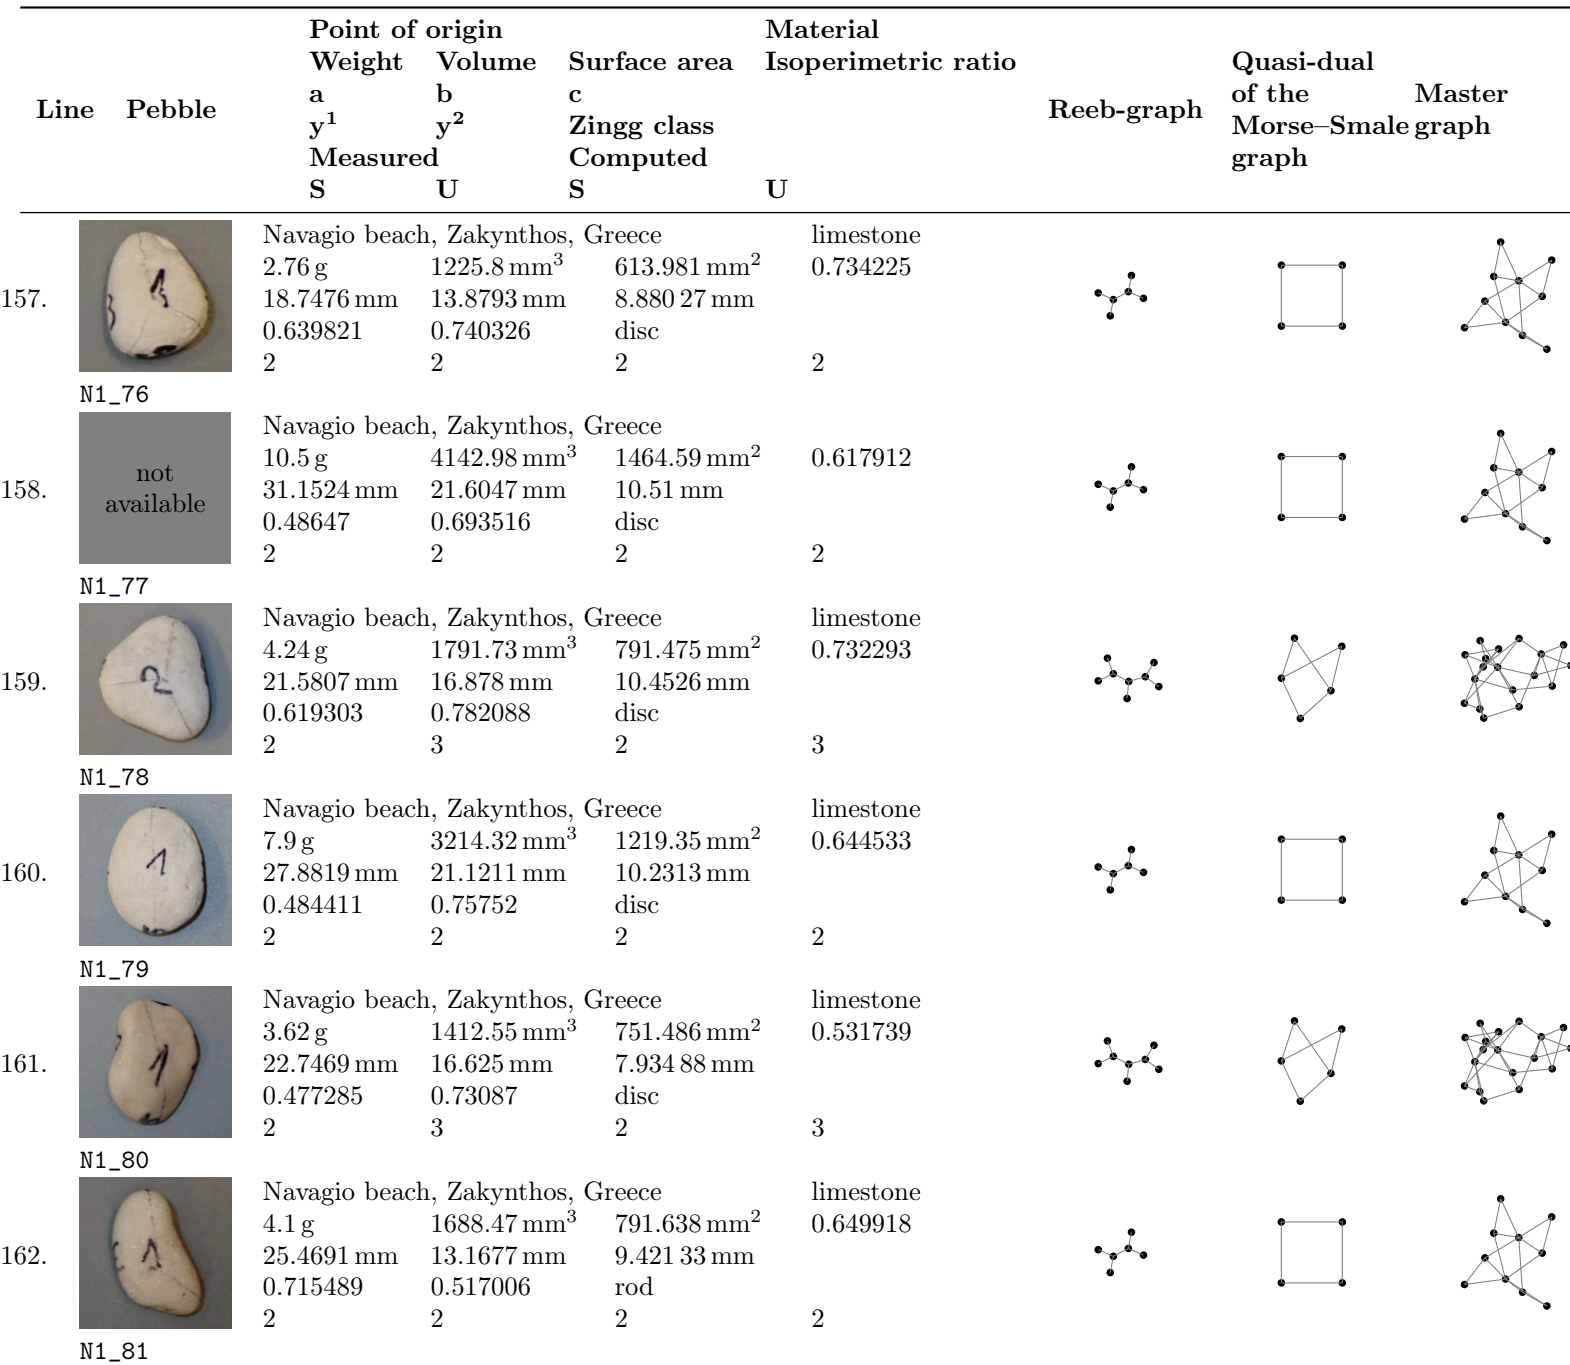   |
|      | N1_77                                                                               |                                                                           |                                                        |                                                     |                                |                     |                                                                                       |                                                                                       |                                                                                       |
| 159. | 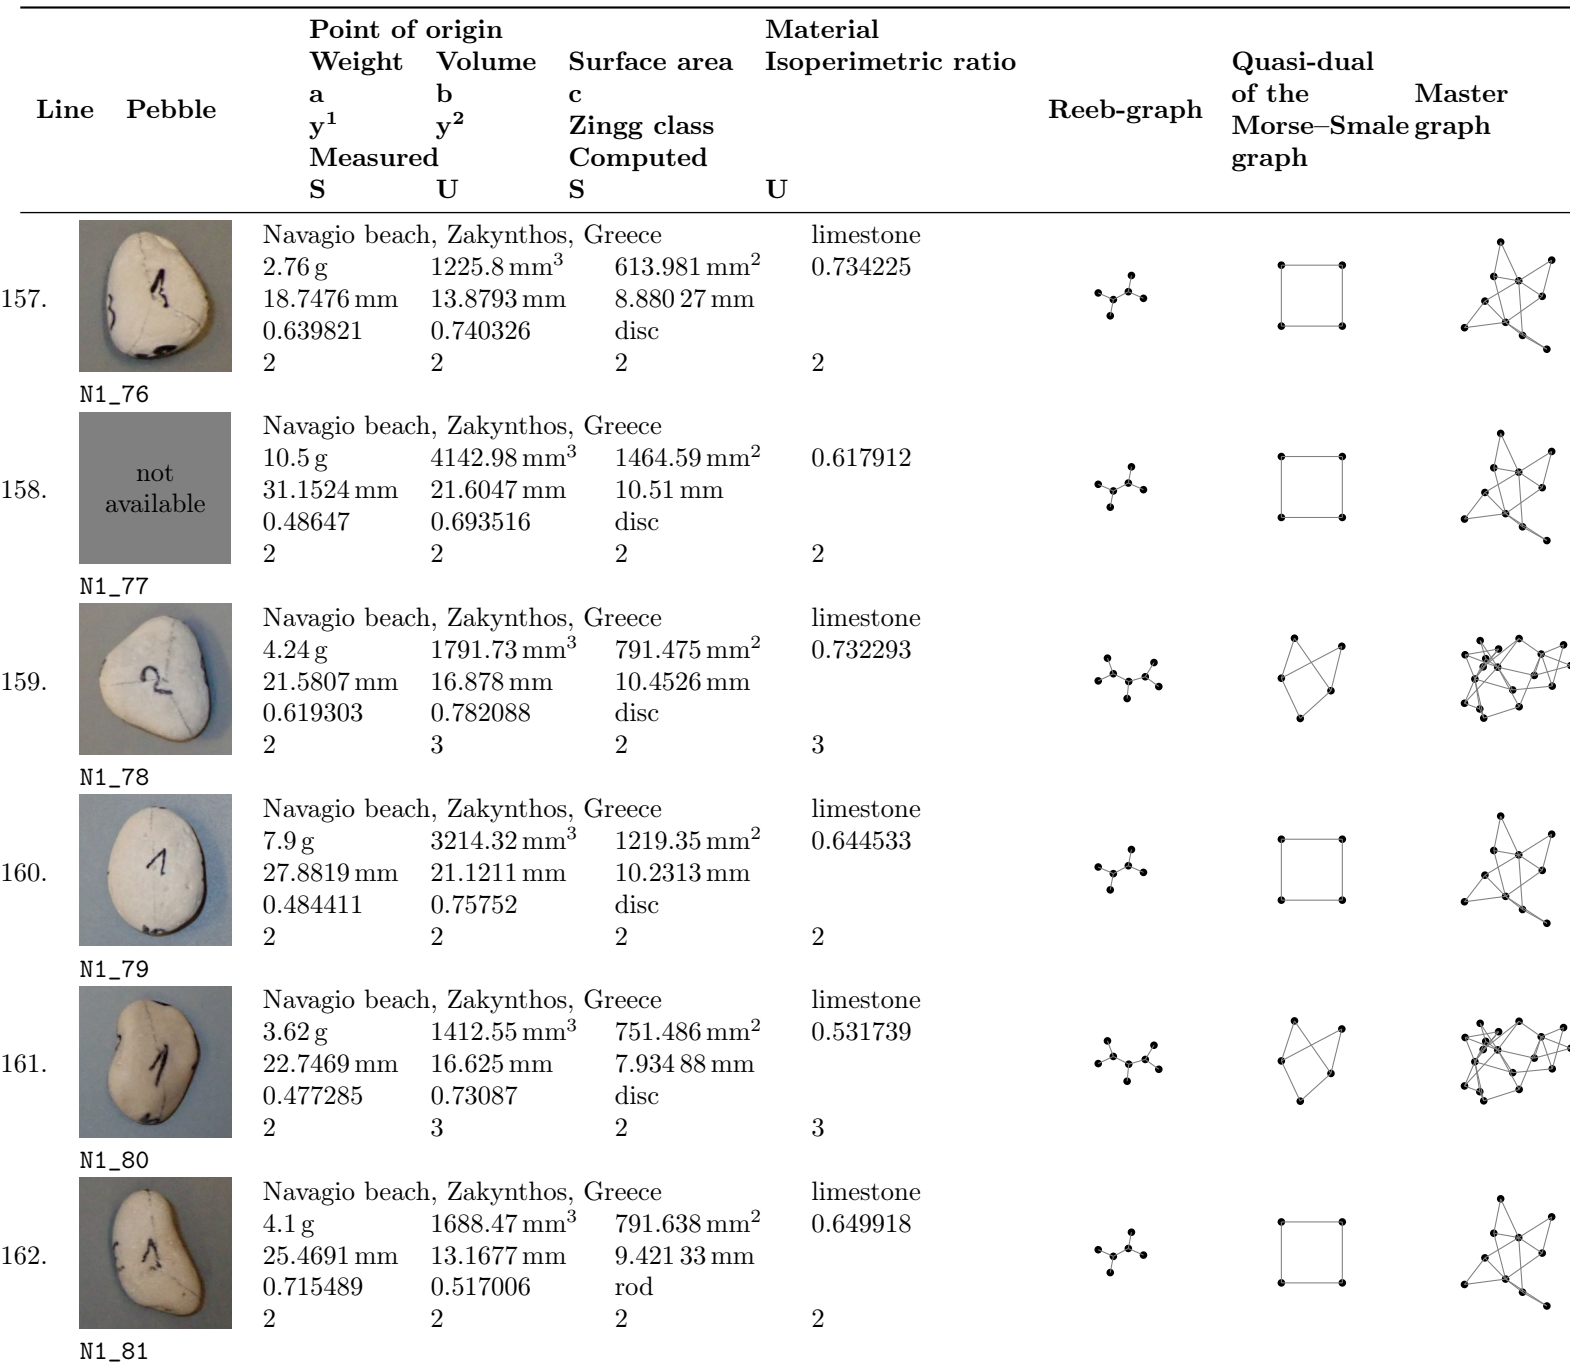   | Navagio beach, Zakynthos, Greece<br>4.24 g<br>21.5807 mm<br>0.619303<br>2 | 1791.73 mm <sup>3</sup><br>16.878 mm<br>0.782088<br>3  | 791.475 mm <sup>2</sup><br>10.4526 mm<br>disc<br>2  | limestone<br>0.732293<br><br>3 |                     | 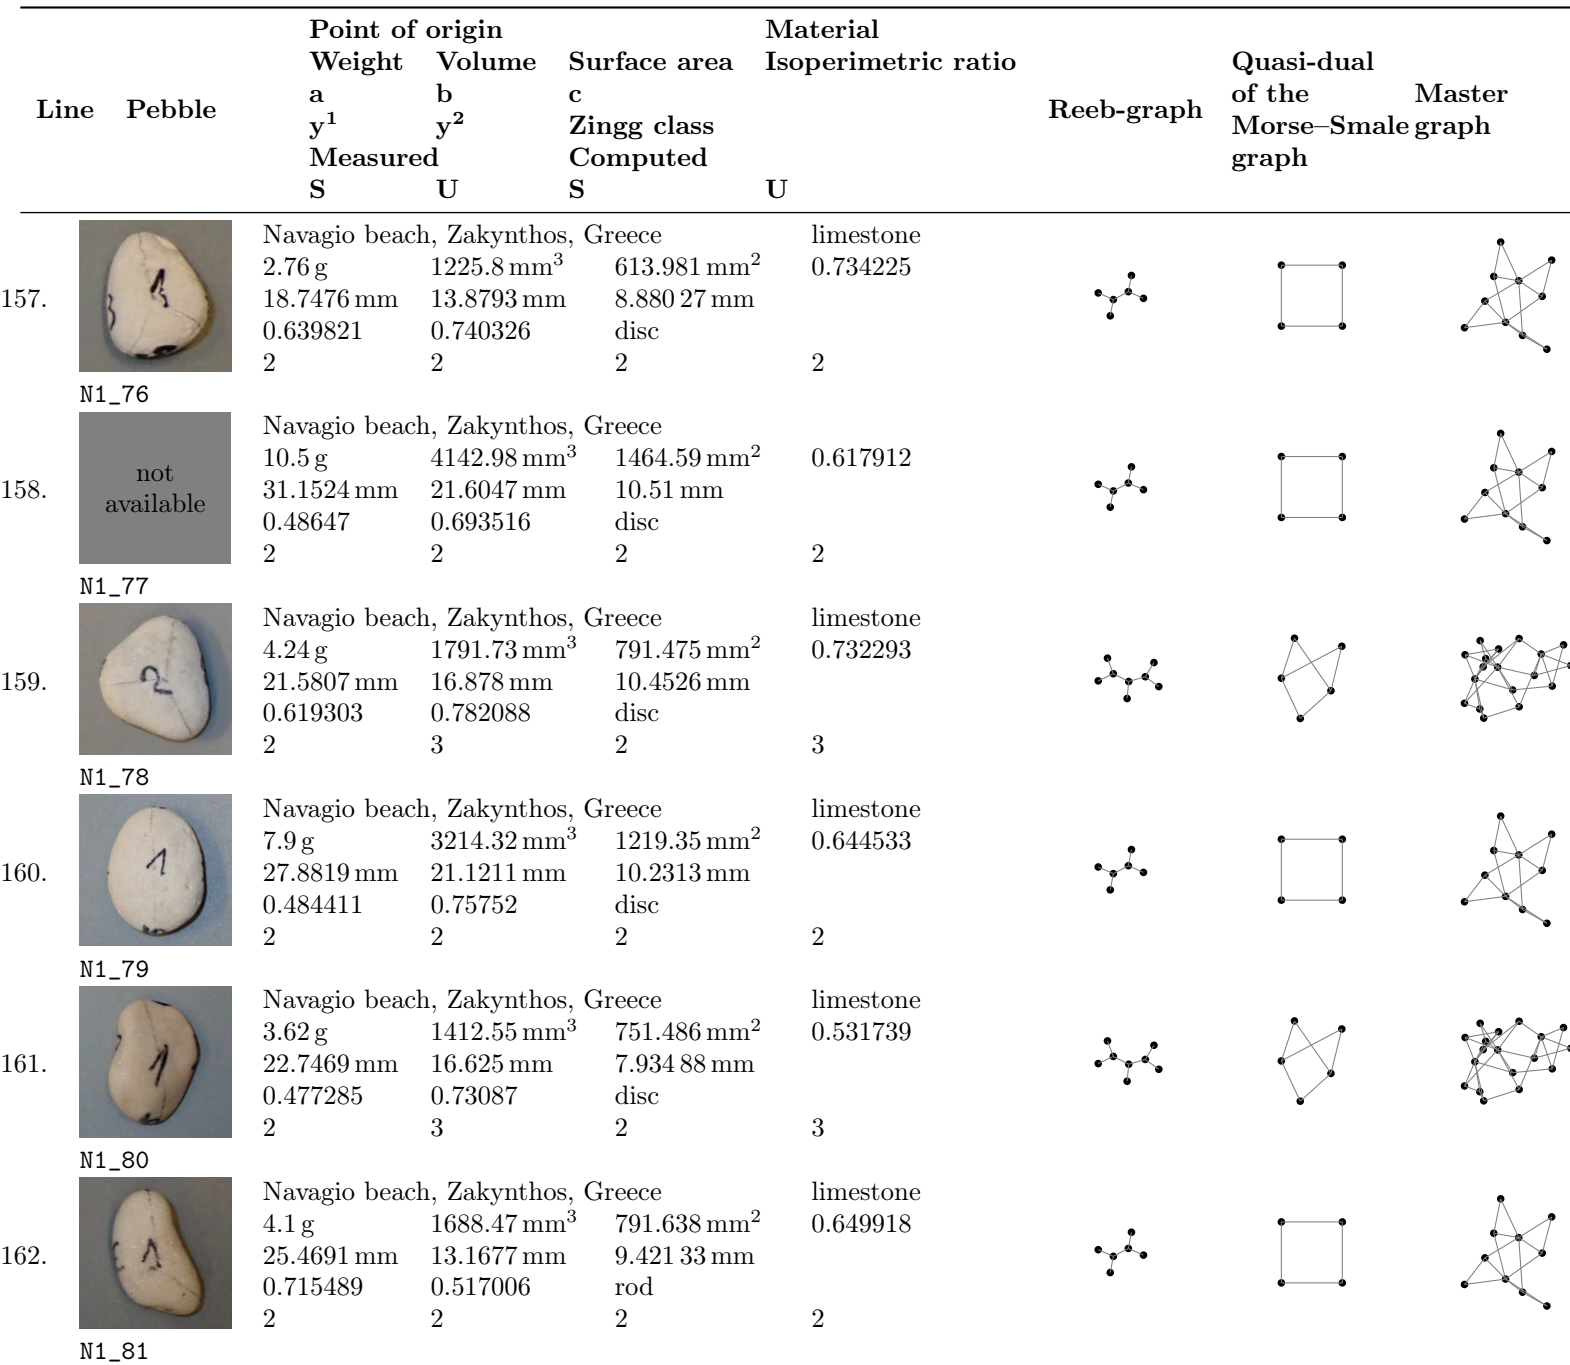   | 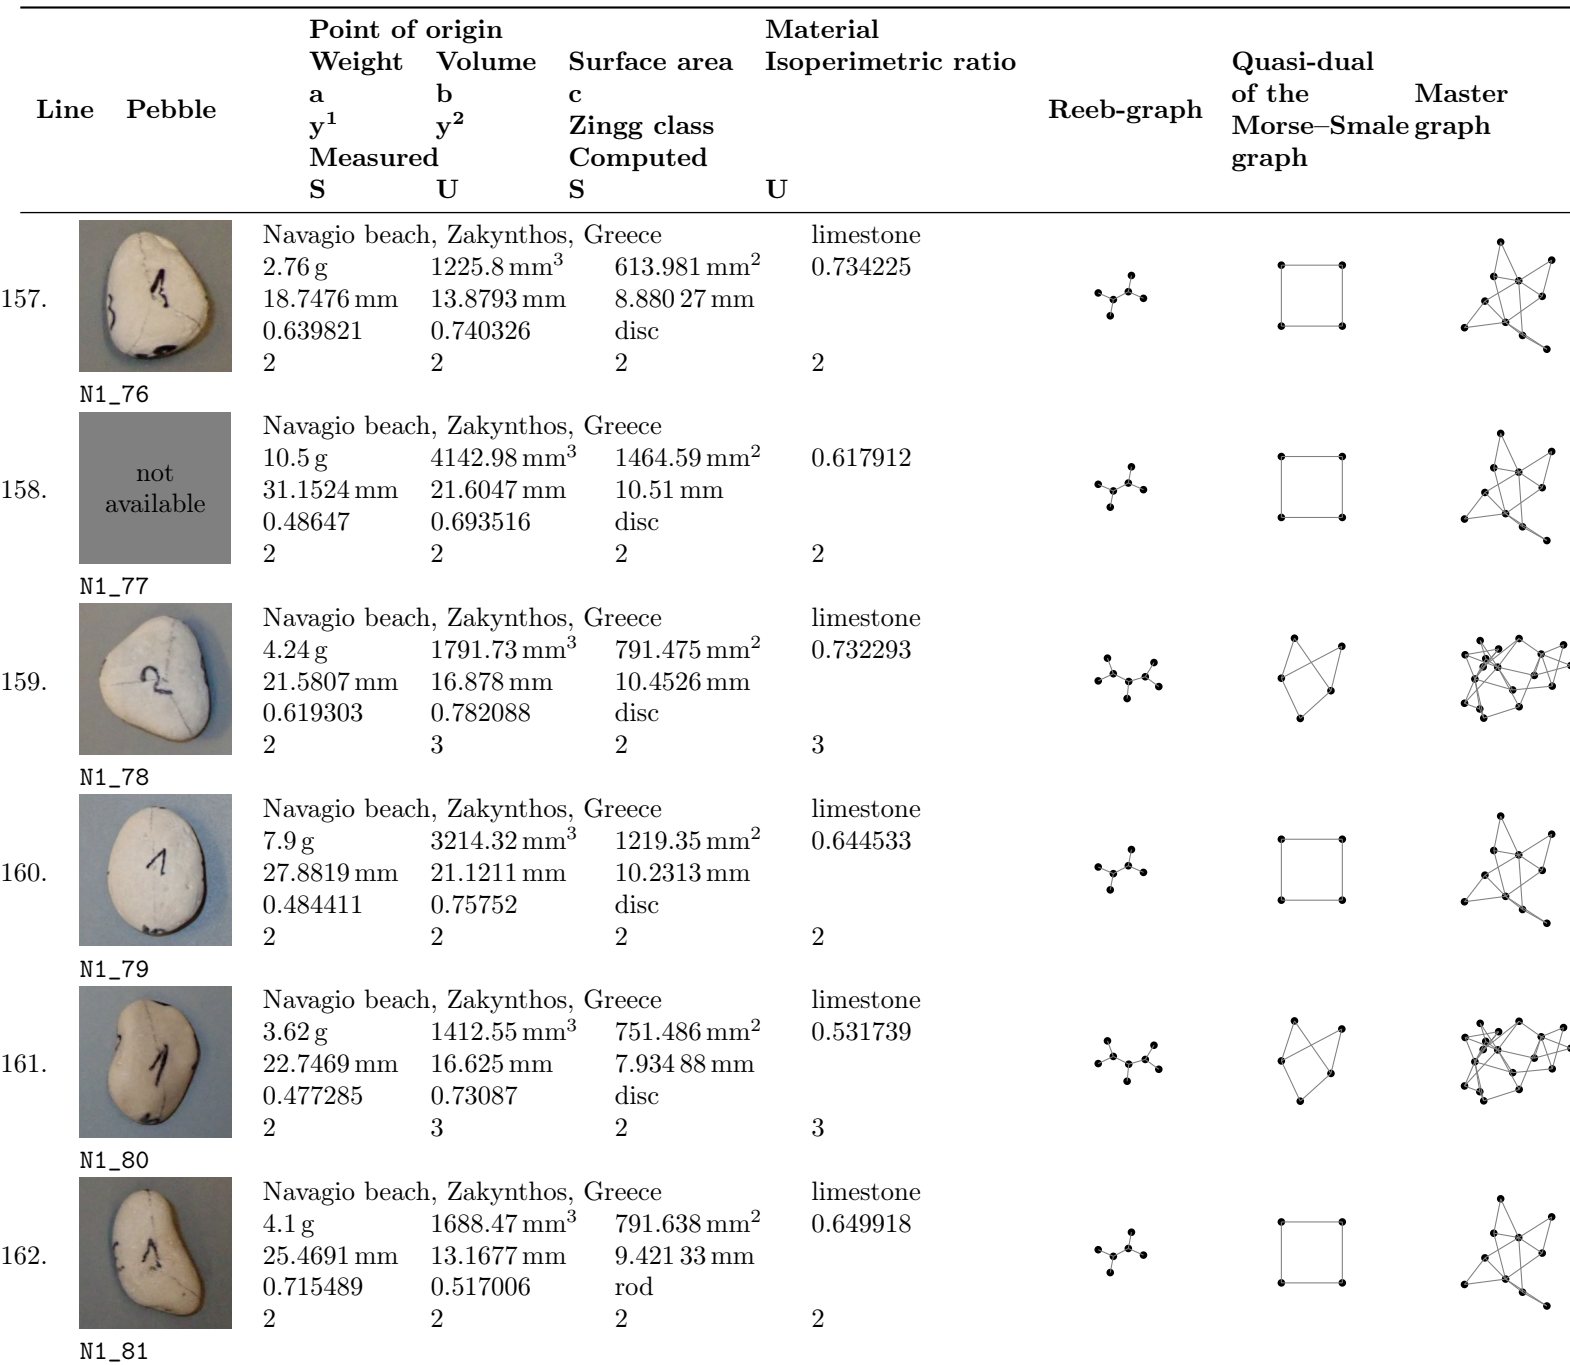   | 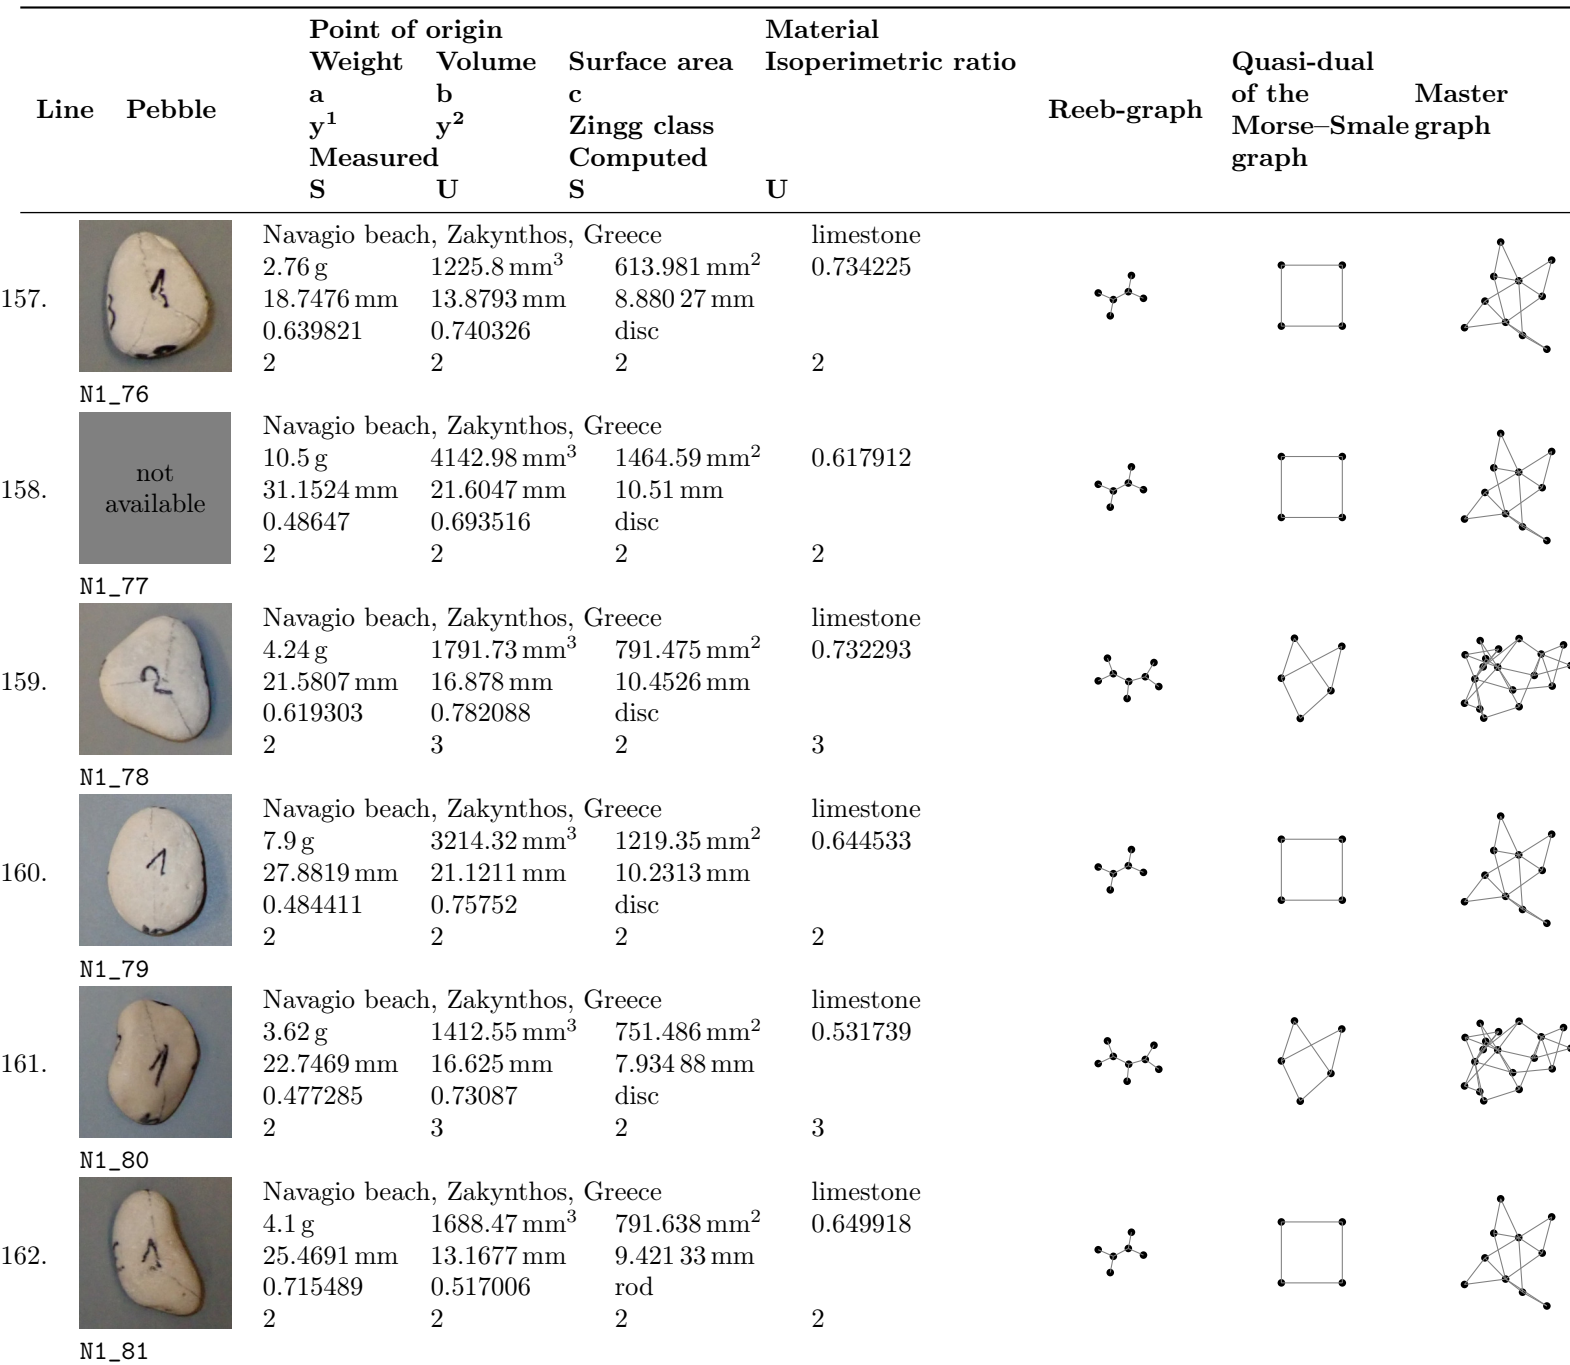   |
|      | N1_78                                                                               |                                                                           |                                                        |                                                     |                                |                     |                                                                                       |                                                                                       |                                                                                       |
| 160. | 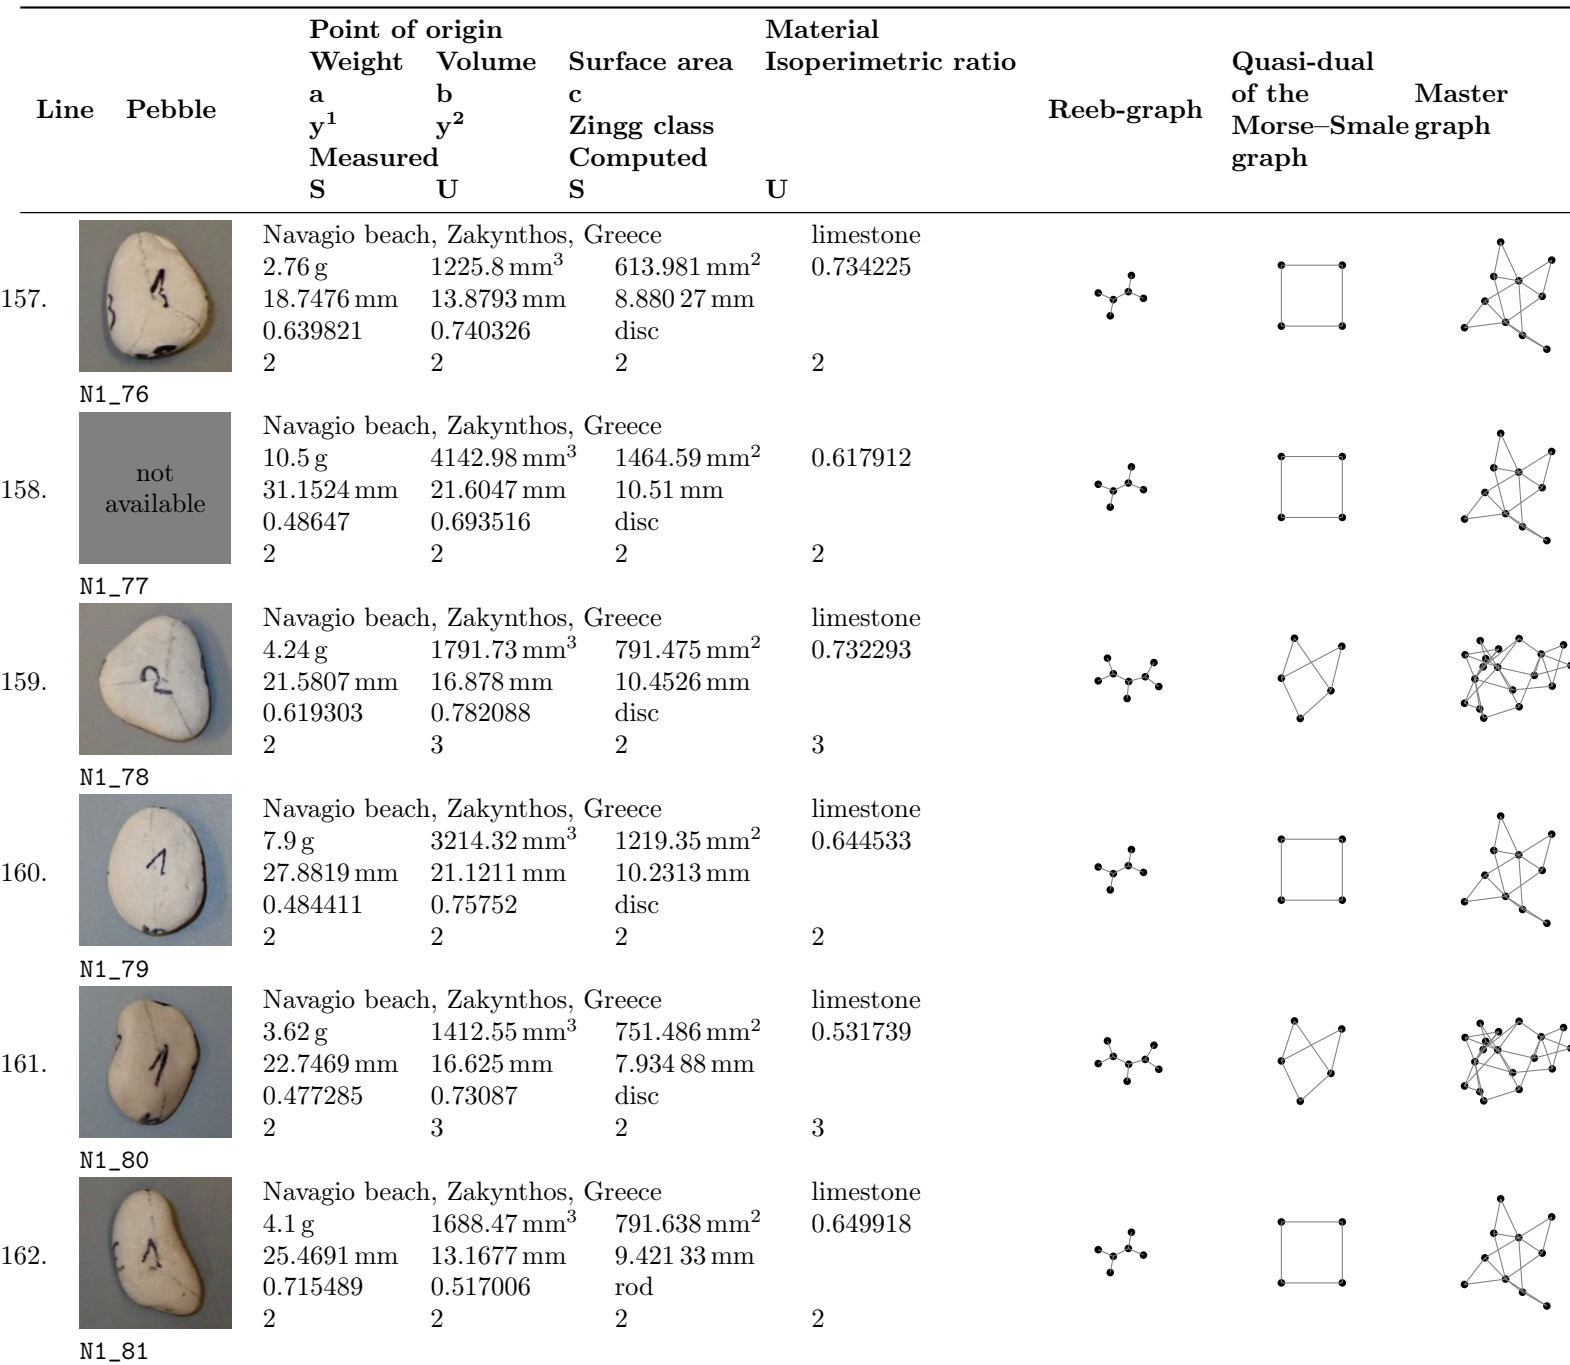  | Navagio beach, Zakynthos, Greece<br>7.9 g<br>27.8819 mm<br>0.484411<br>2  | 3214.32 mm <sup>3</sup><br>21.1211 mm<br>0.75752<br>2  | 1219.35 mm <sup>2</sup><br>10.2313 mm<br>disc<br>2  | limestone<br>0.644533<br><br>2 |                     | 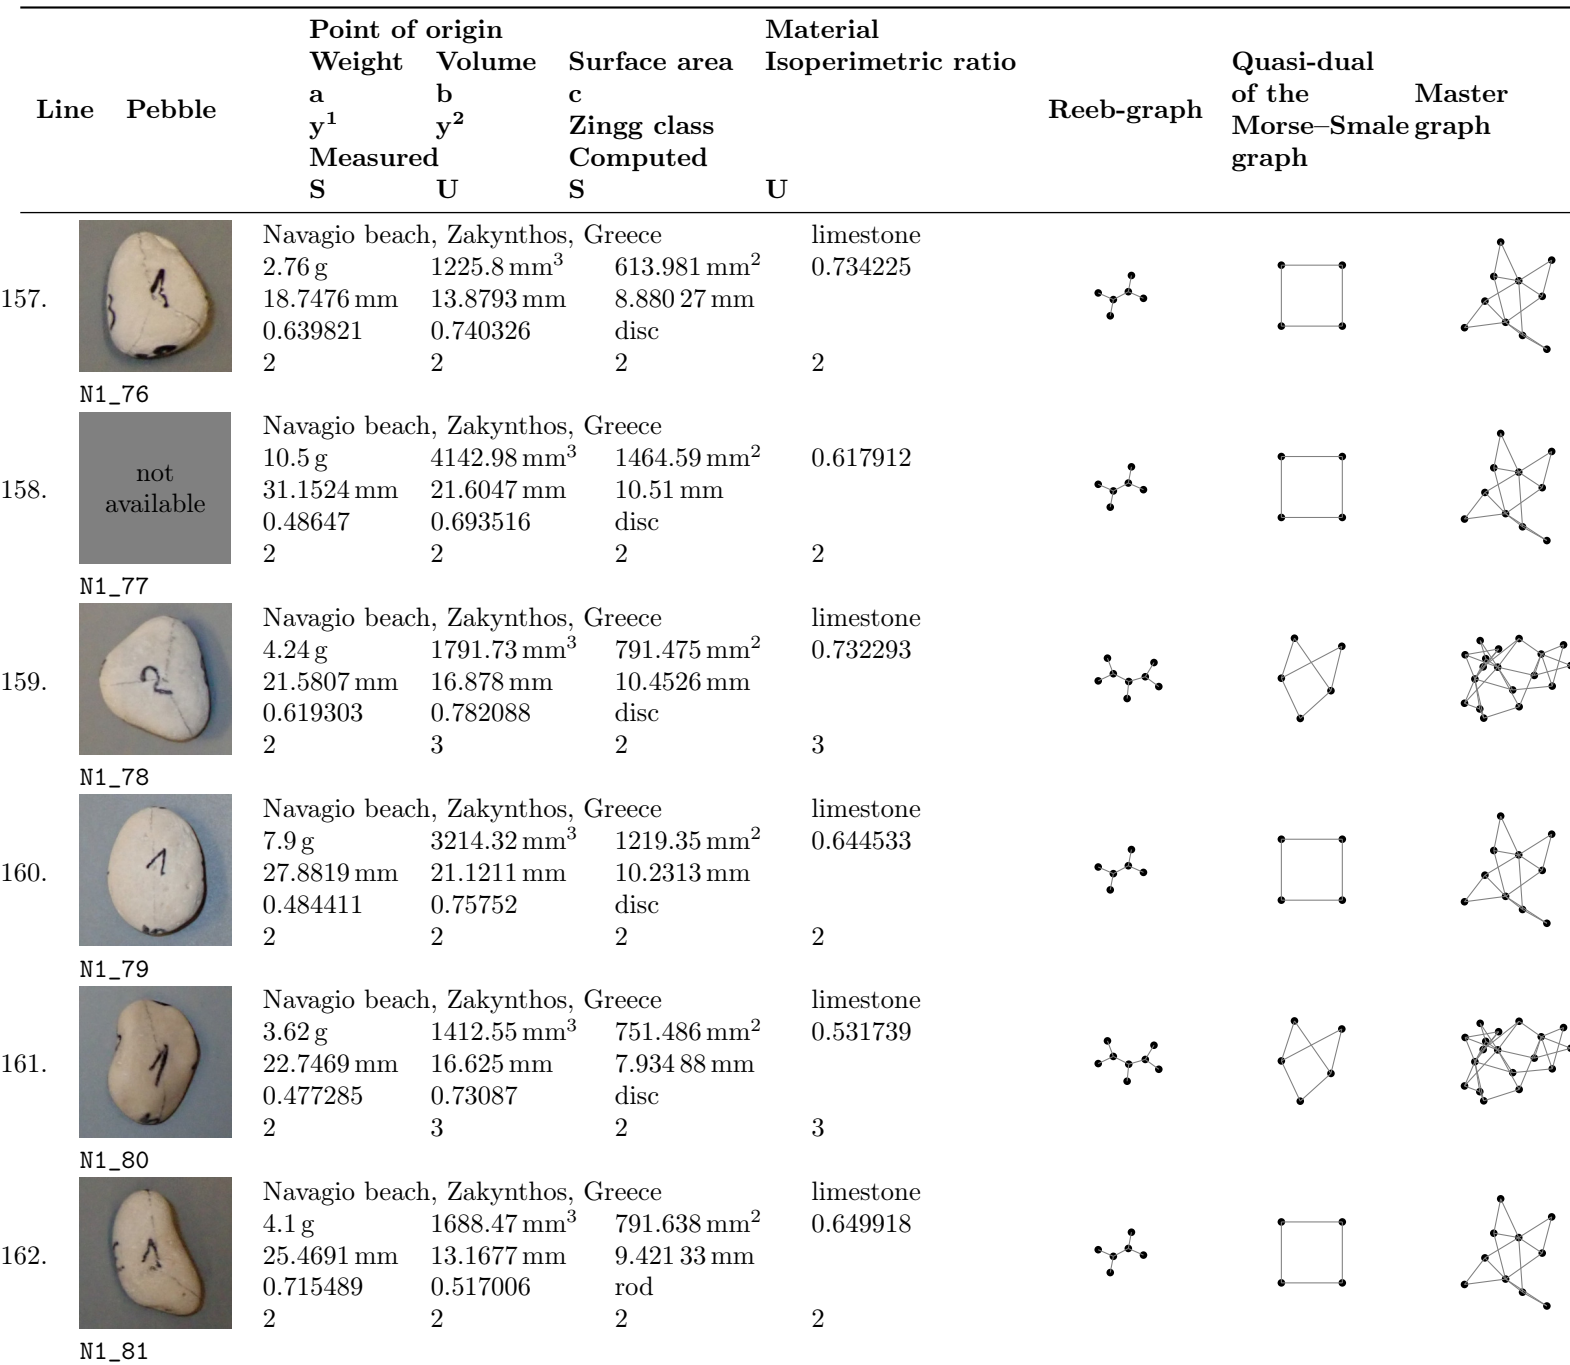  | 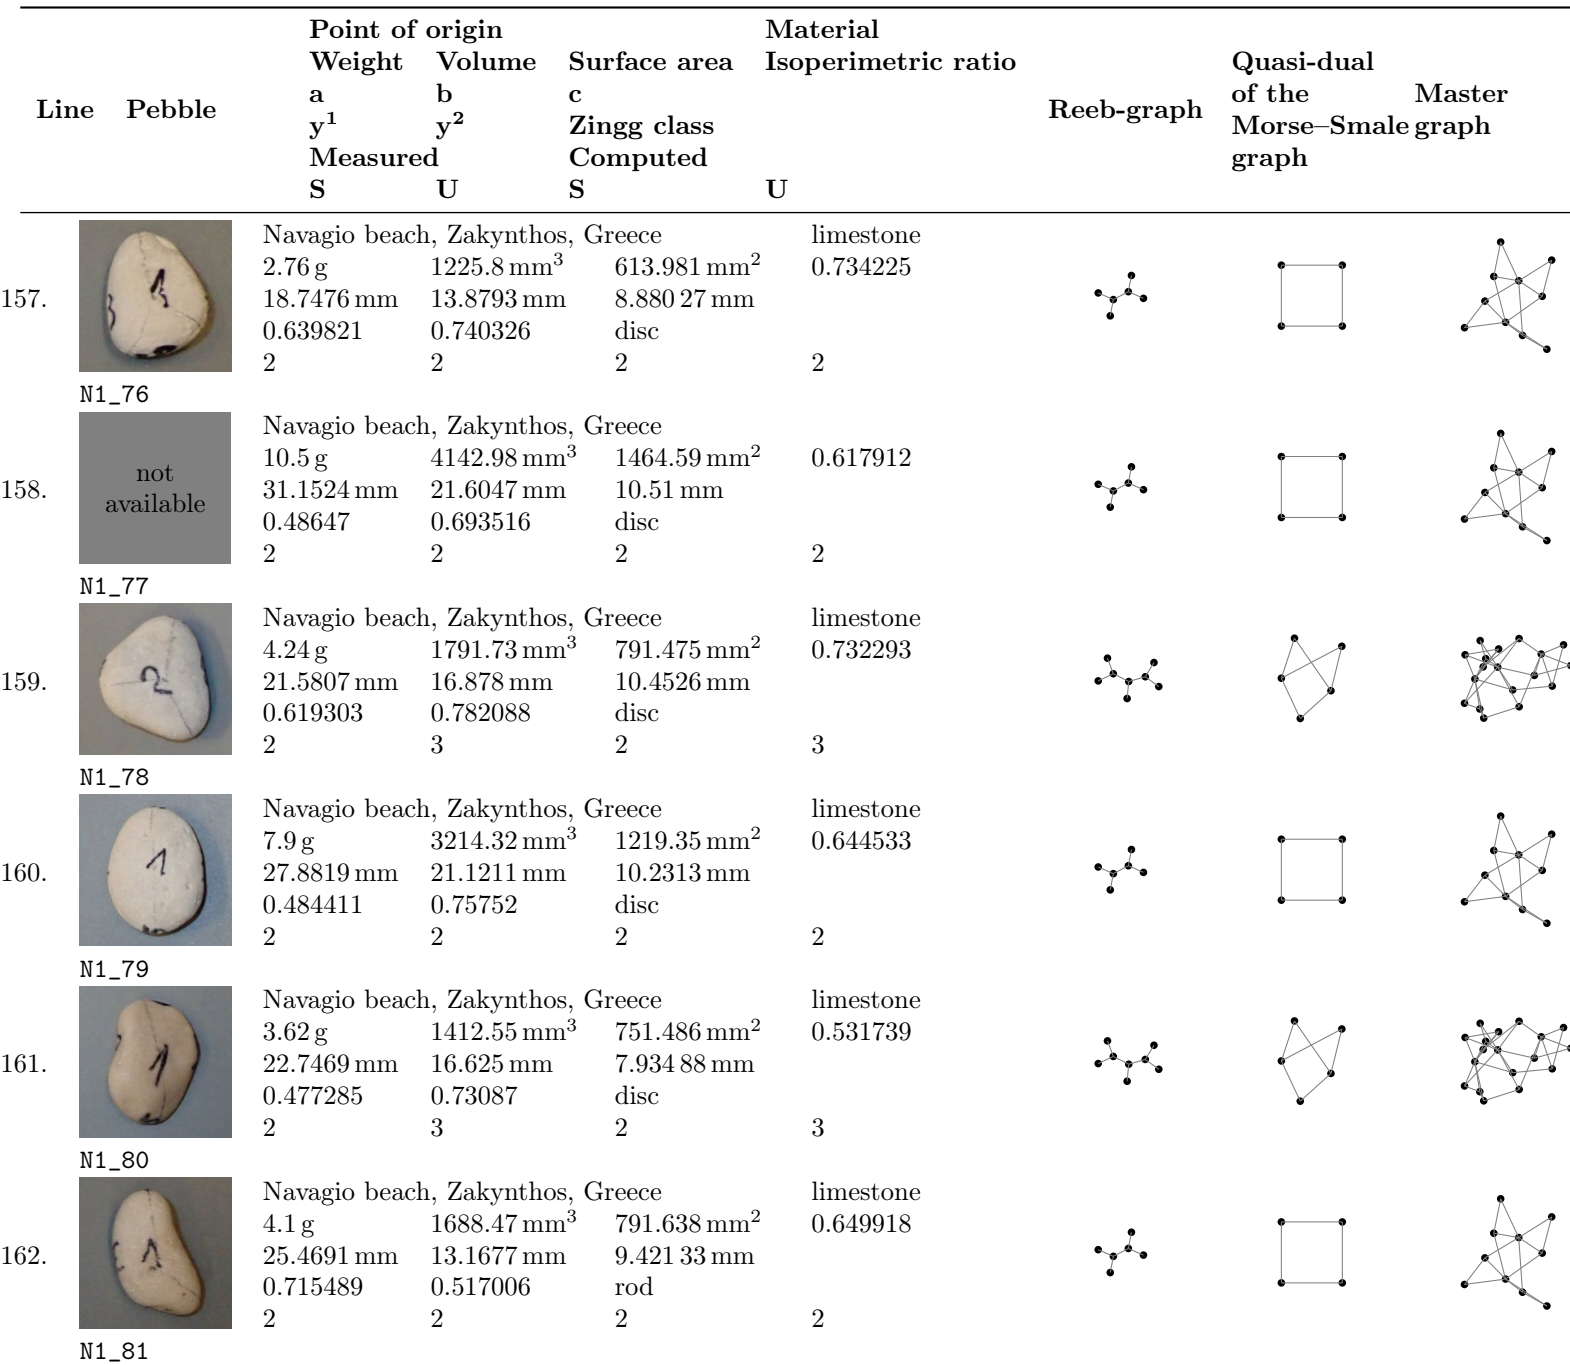  | 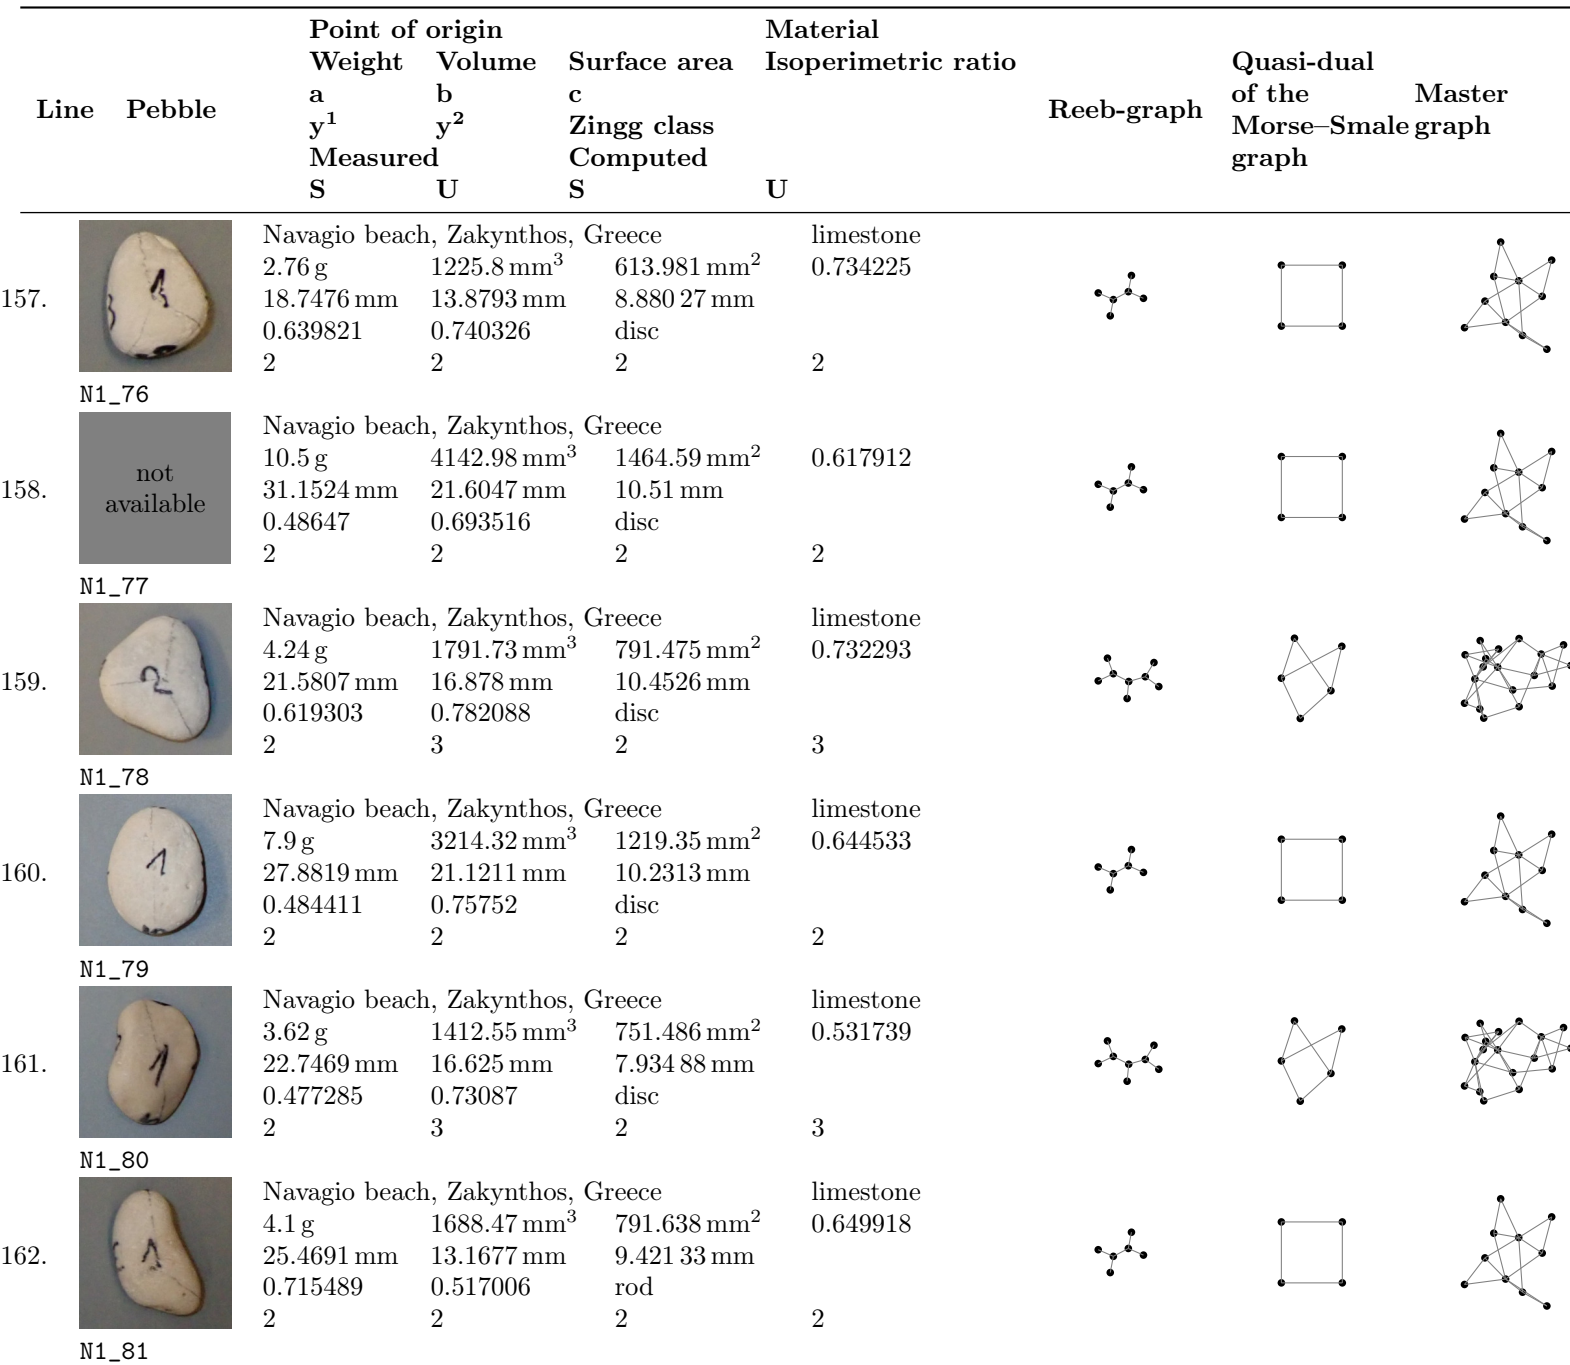  |
|      | N1_79                                                                               |                                                                           |                                                        |                                                     |                                |                     |                                                                                       |                                                                                       |                                                                                       |
| 161. | 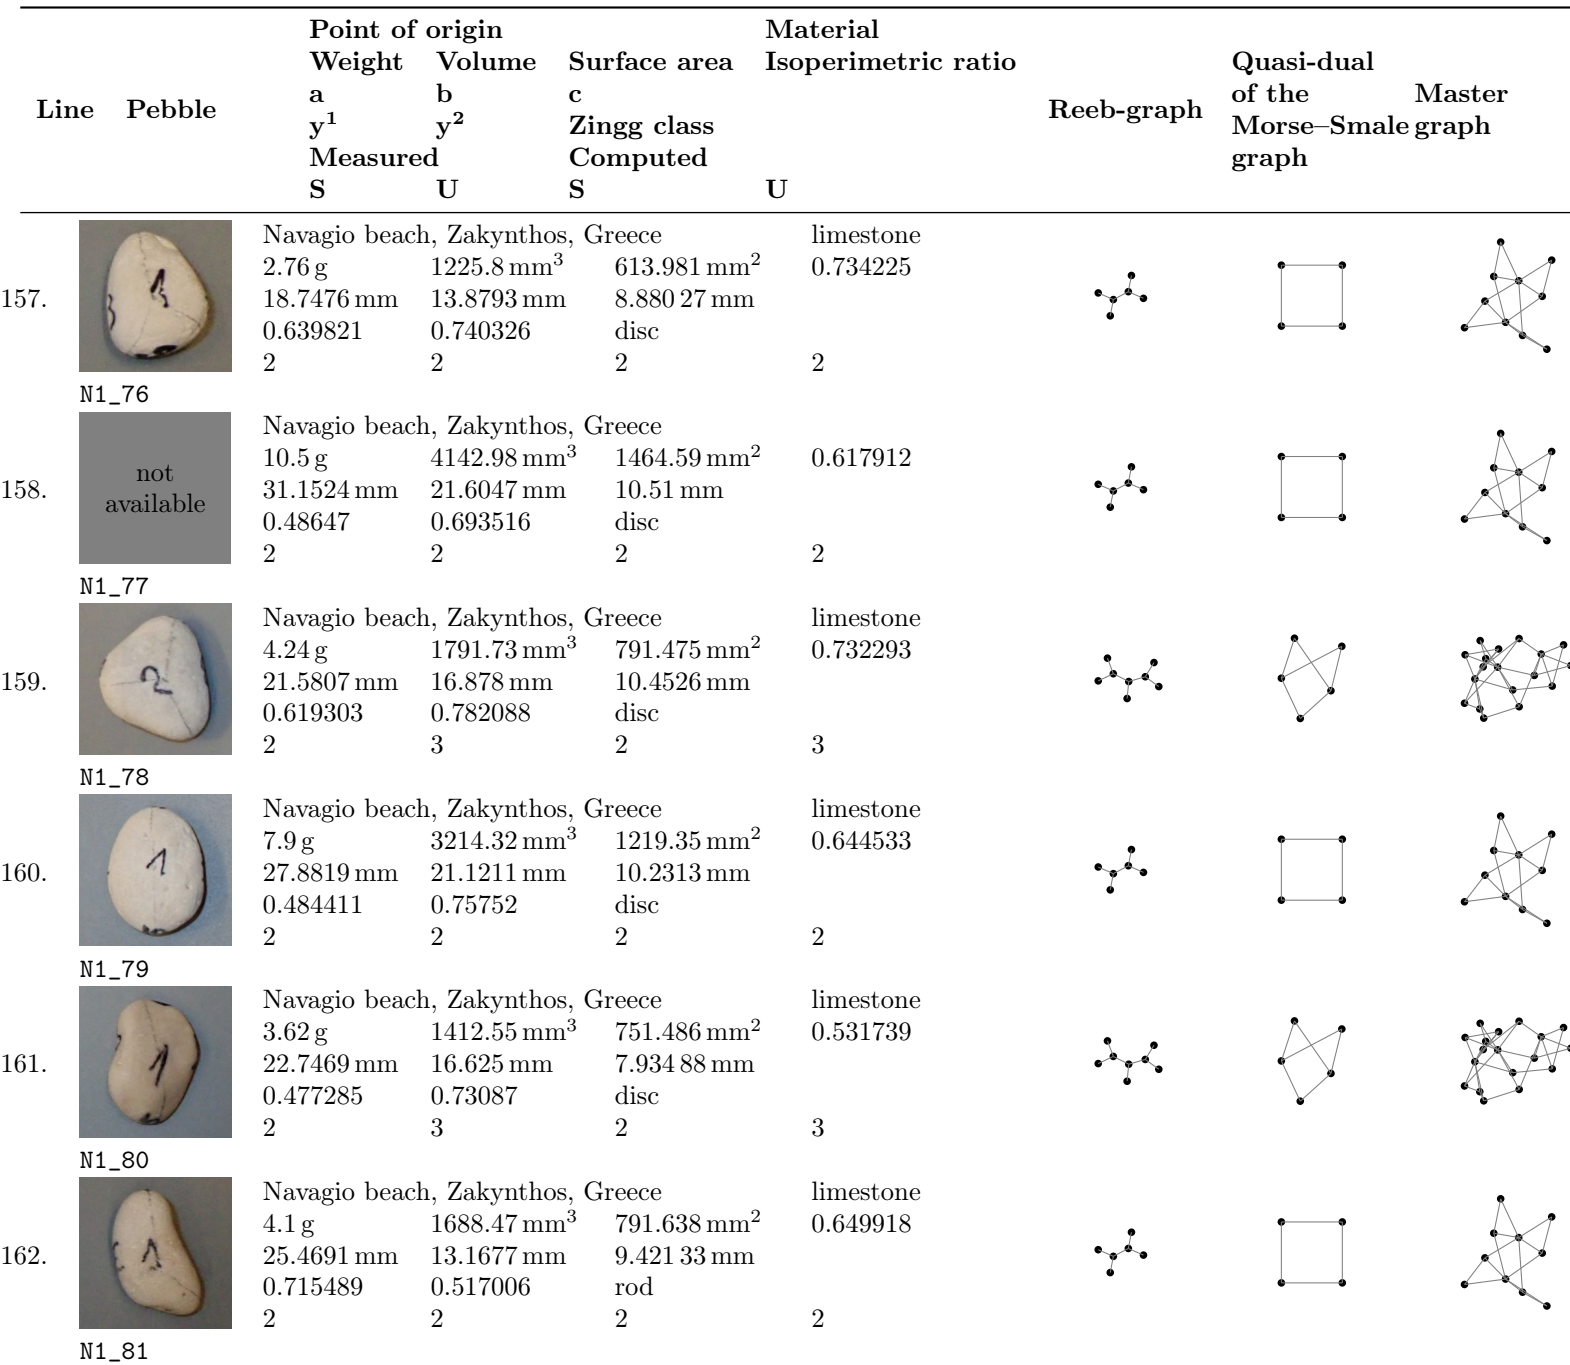 | Navagio beach, Zakynthos, Greece<br>3.62 g<br>22.7469 mm<br>0.477285<br>2 | 1412.55 mm <sup>3</sup><br>16.625 mm<br>0.73087<br>3   | 751.486 mm <sup>2</sup><br>7.934 88 mm<br>disc<br>2 | limestone<br>0.531739<br><br>3 |                     | 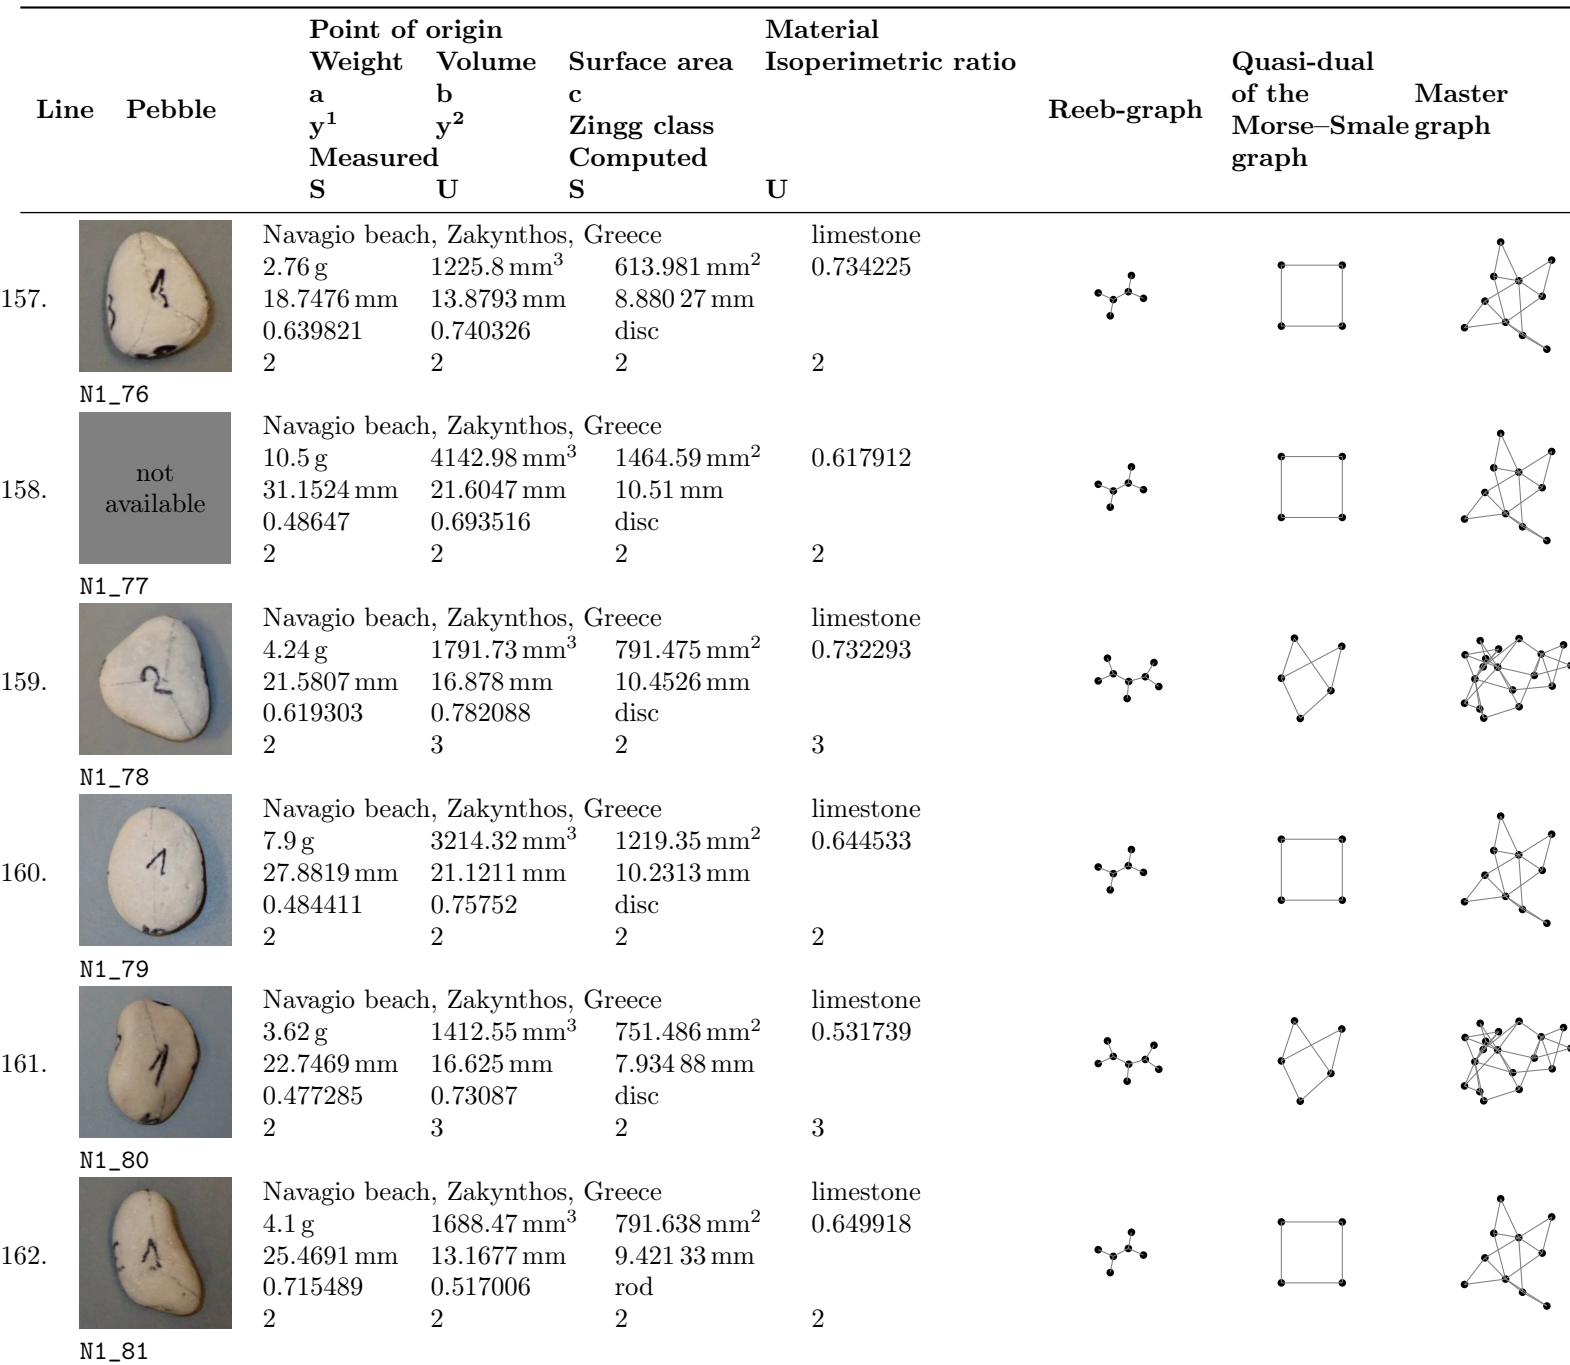 | 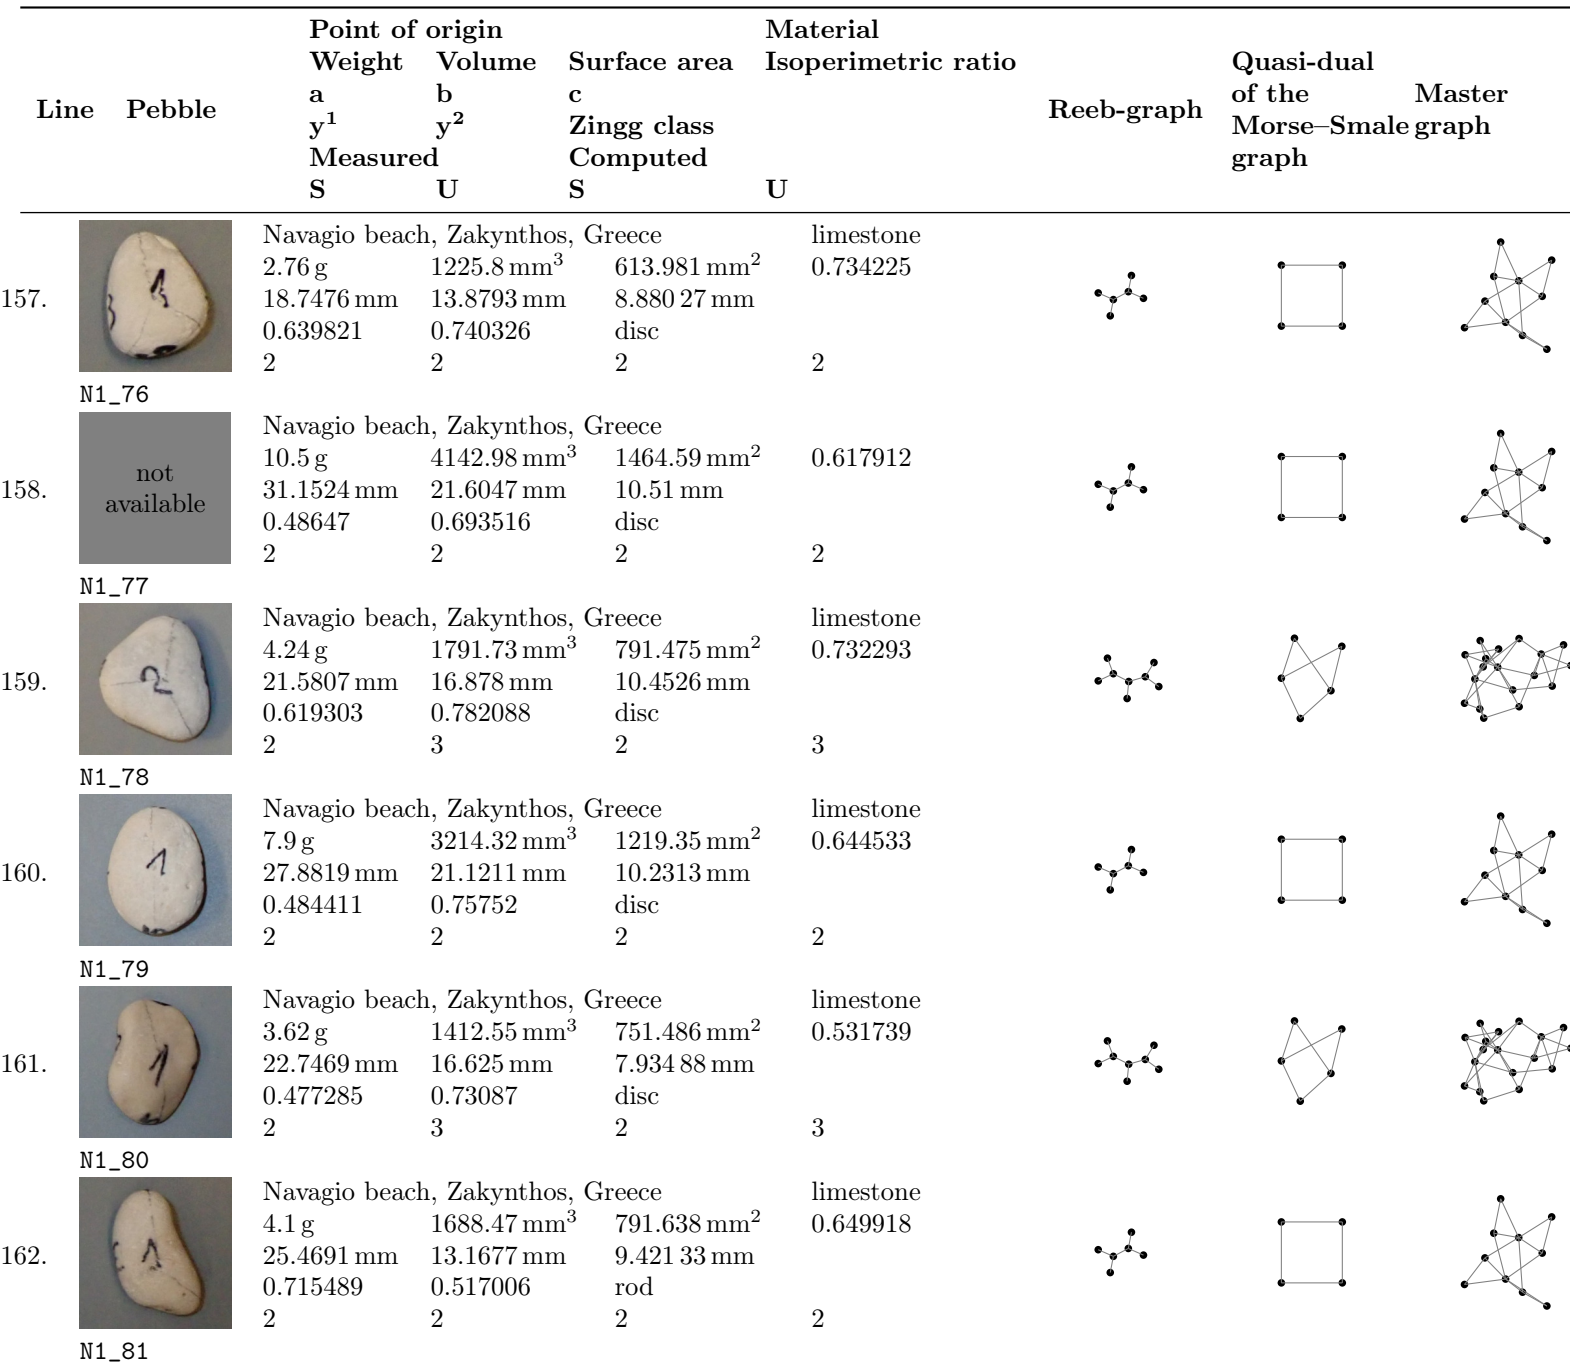 | 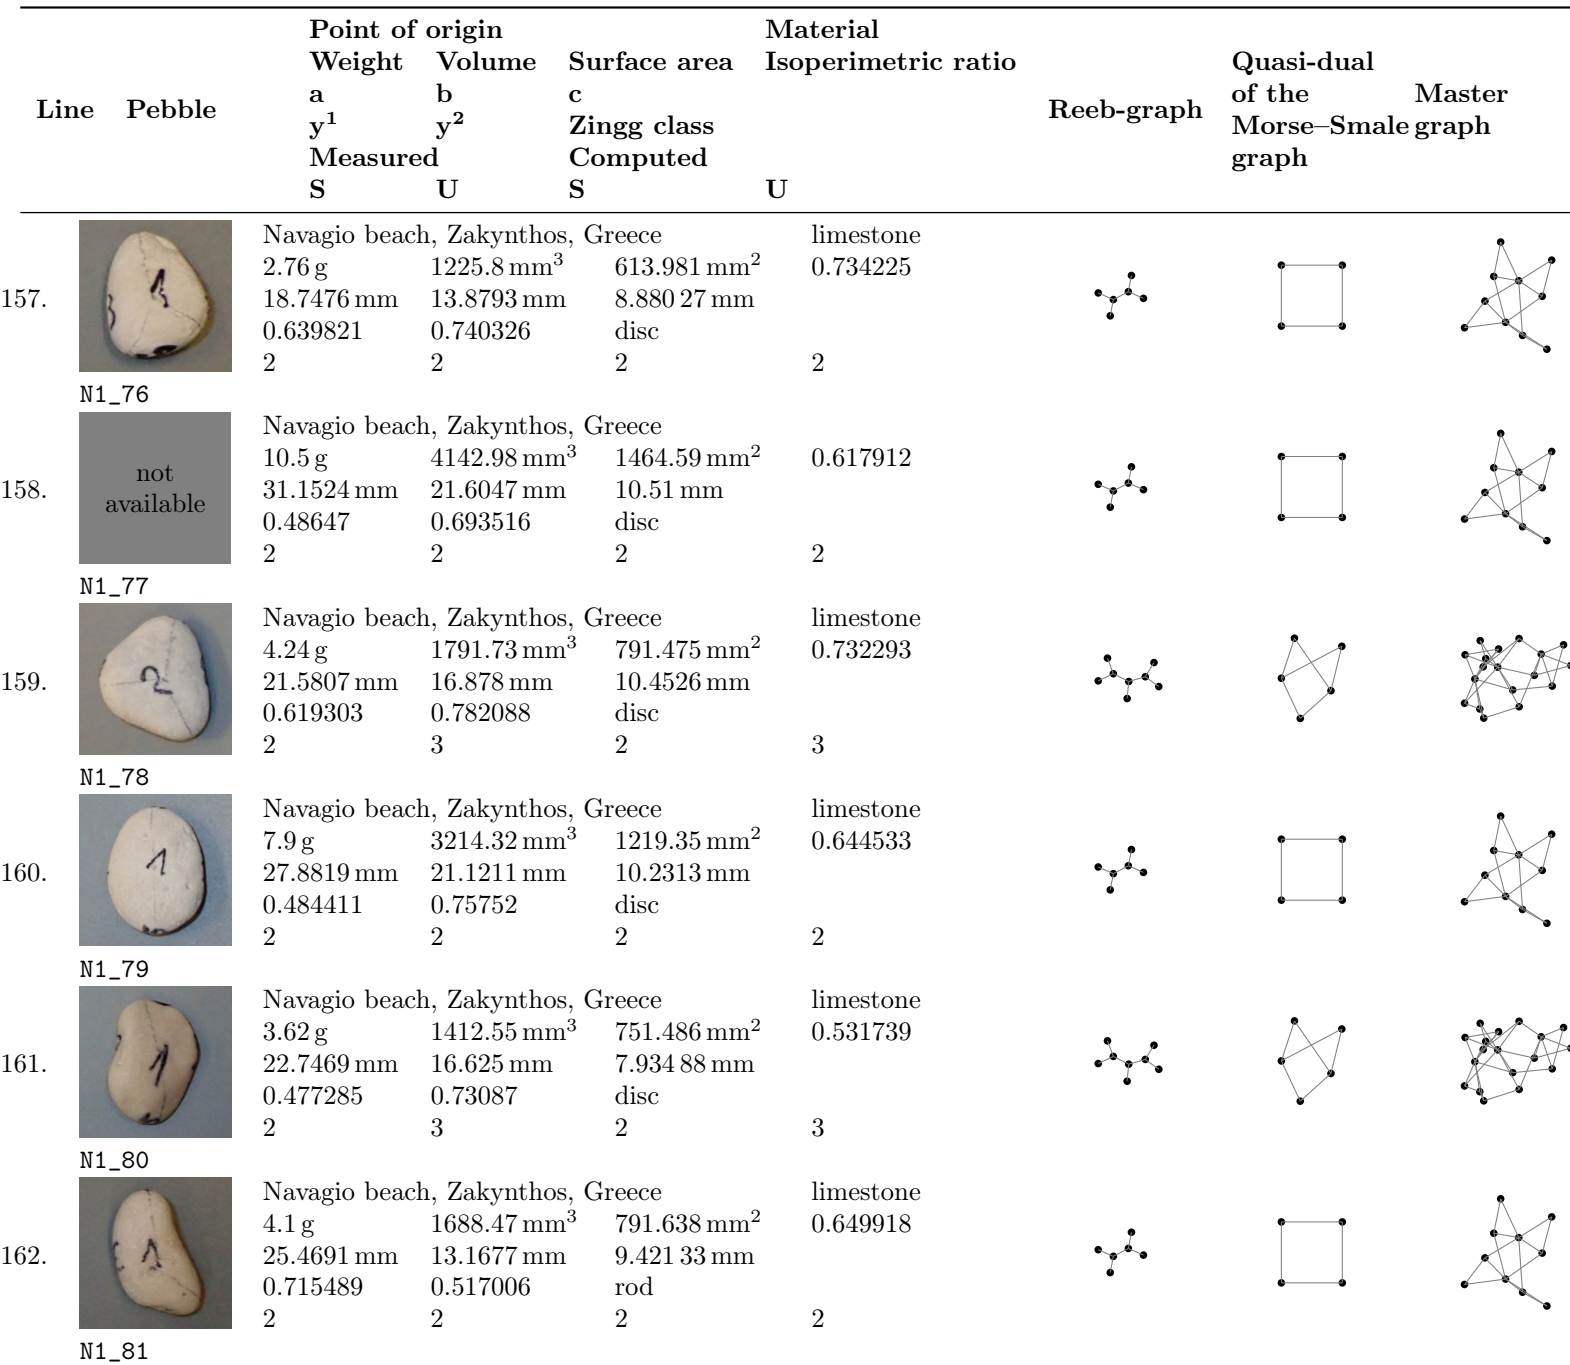 |
|      | N1_80                                                                               |                                                                           |                                                        |                                                     |                                |                     |                                                                                       |                                                                                       |                                                                                       |
| 162. | 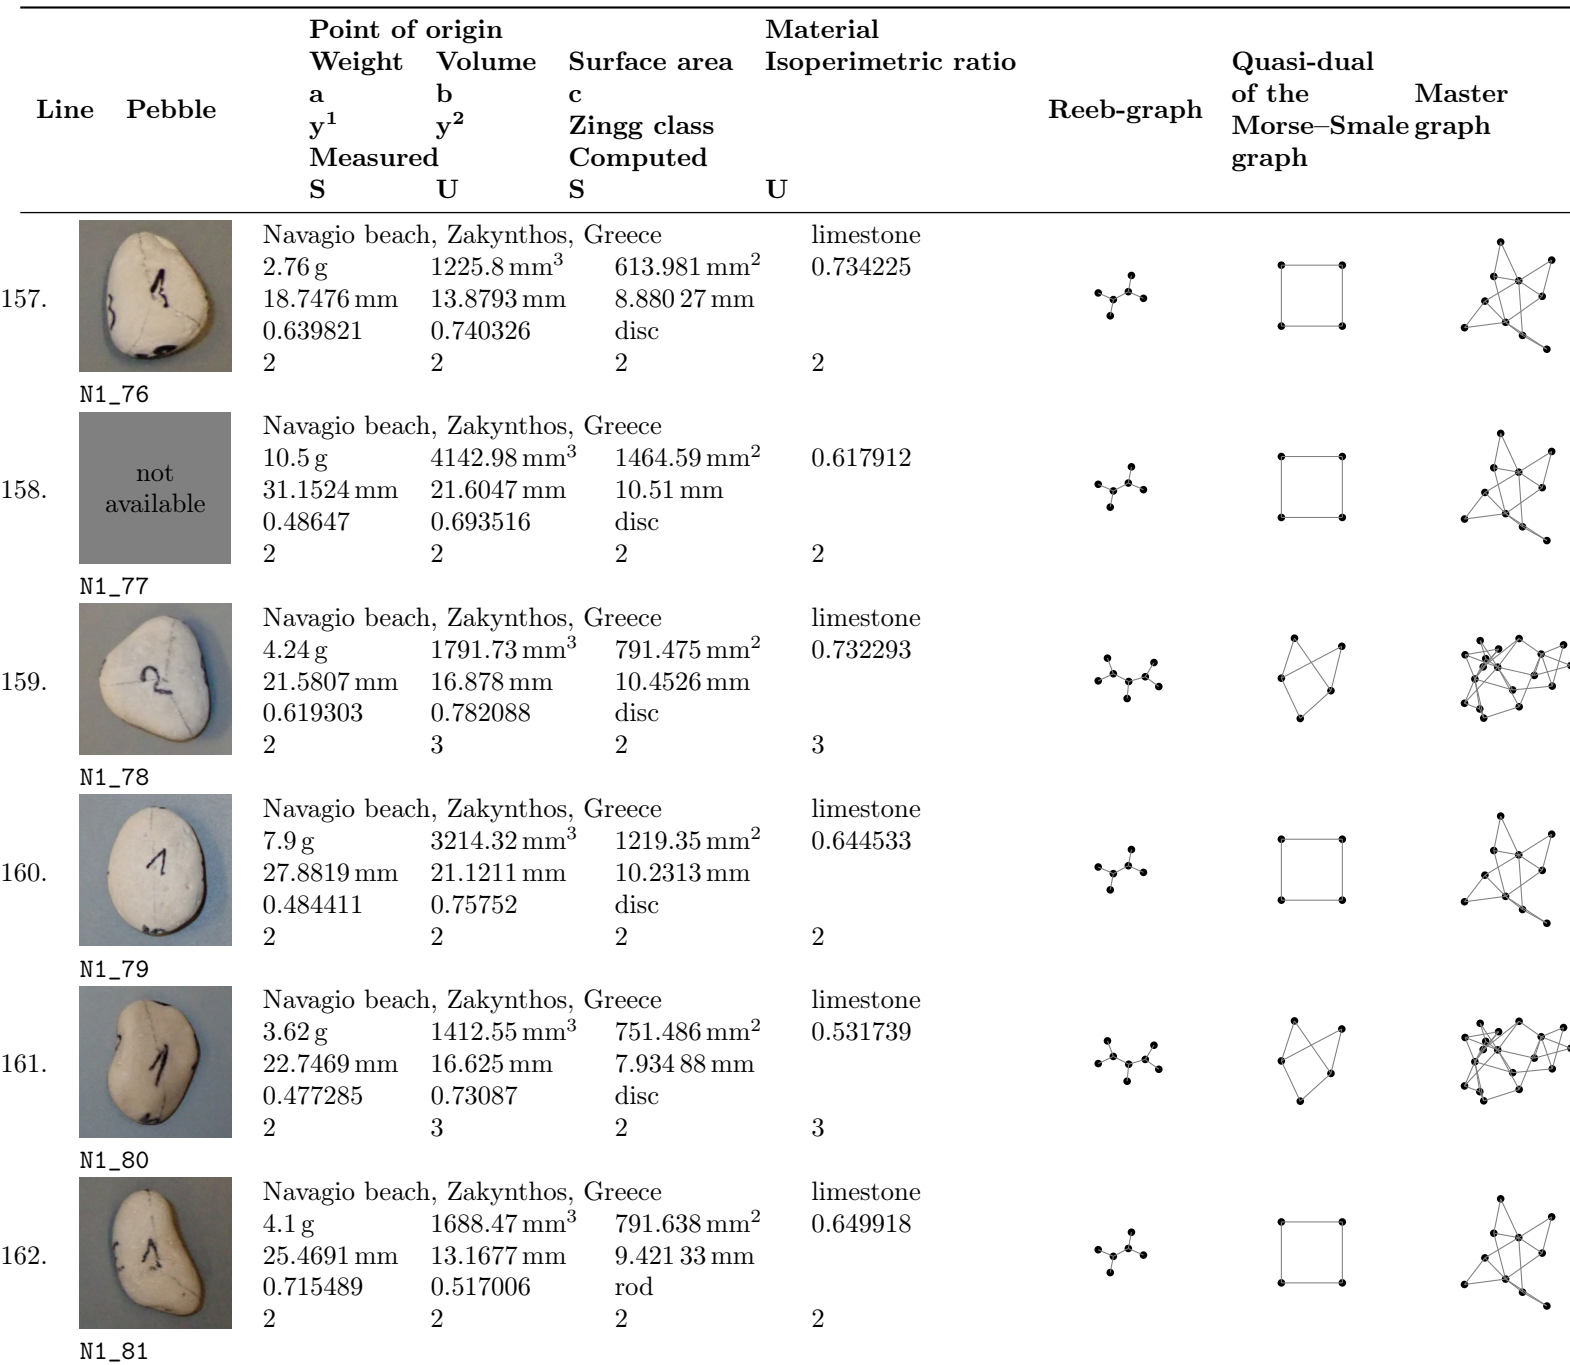 | Navagio beach, Zakynthos, Greece<br>4.1 g<br>25.4691 mm<br>0.715489<br>2  | 1688.47 mm <sup>3</sup><br>13.1677 mm<br>0.517006<br>2 | 791.638 mm <sup>2</sup><br>9.421 33 mm<br>rod<br>2  | limestone<br>0.649918<br><br>2 |                     | 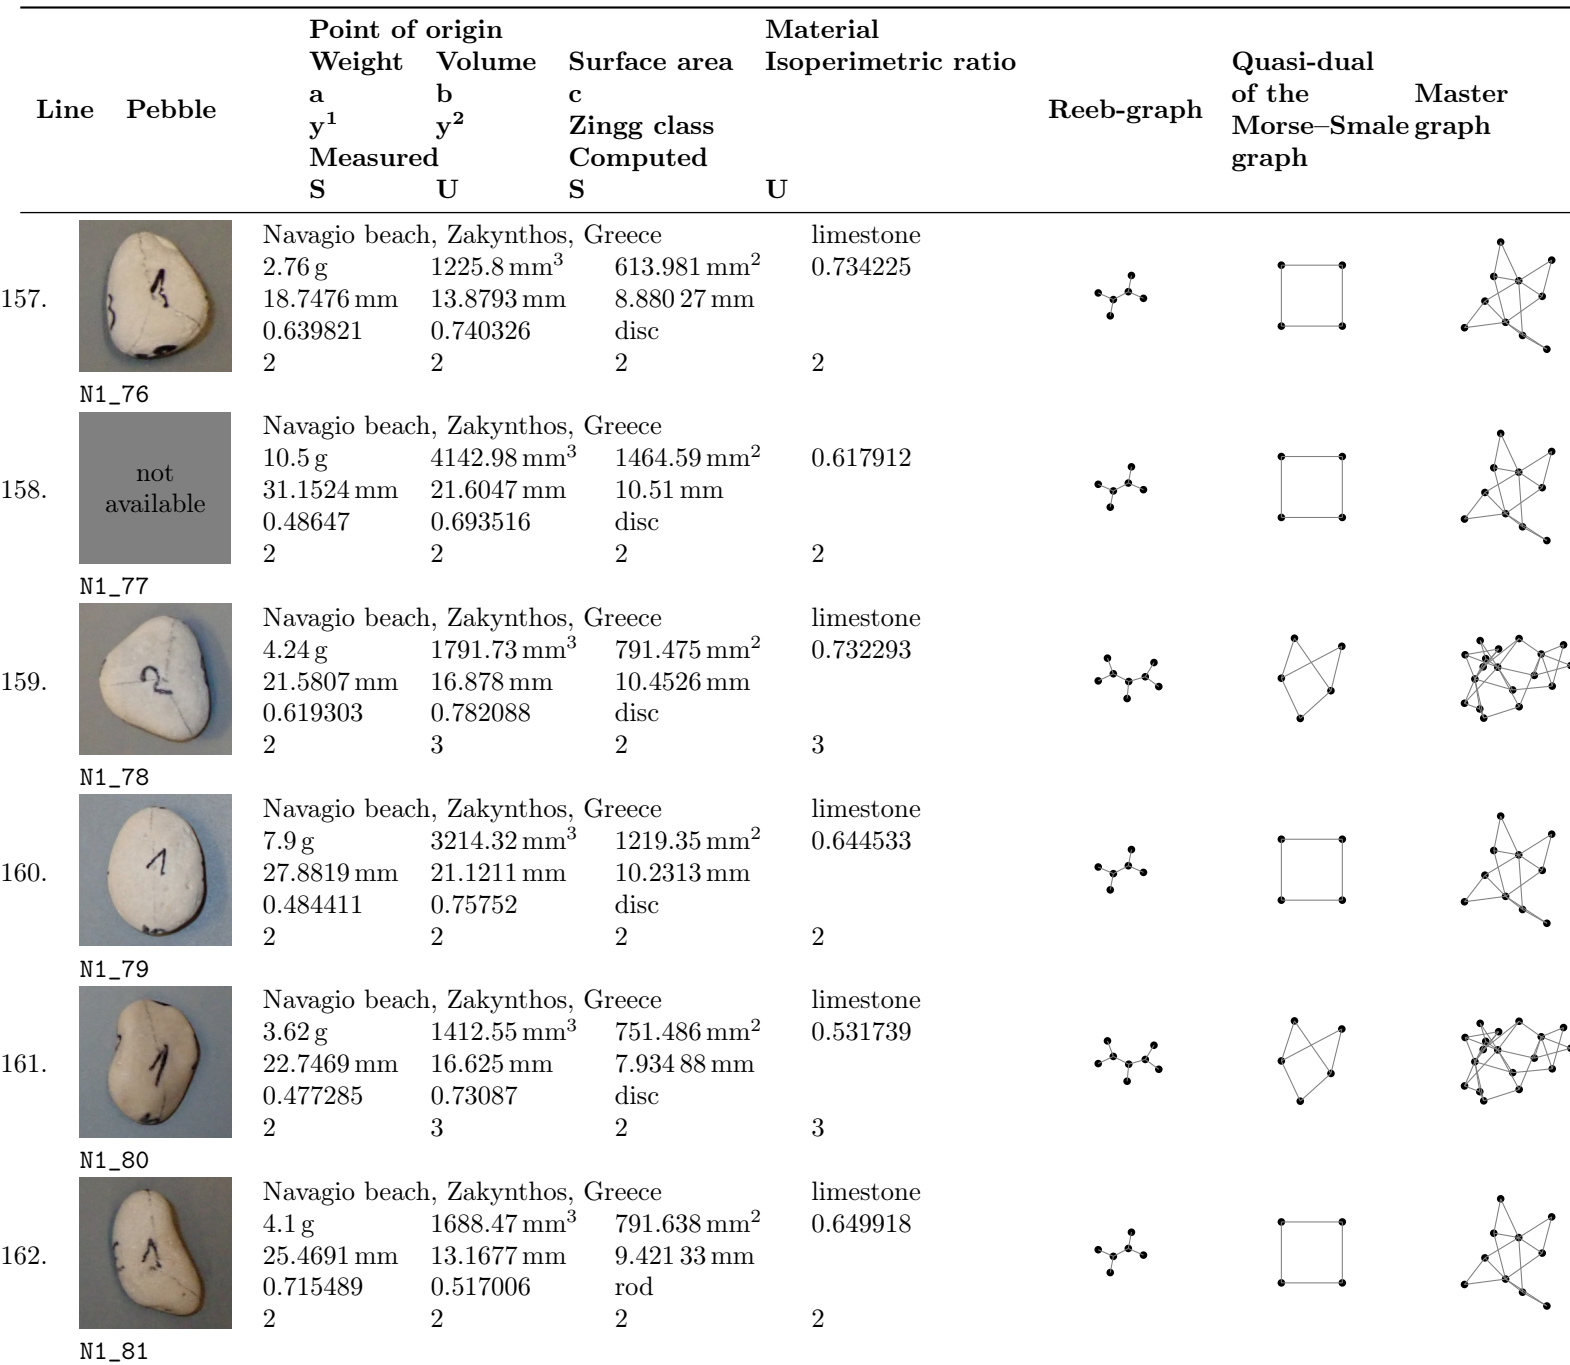 | 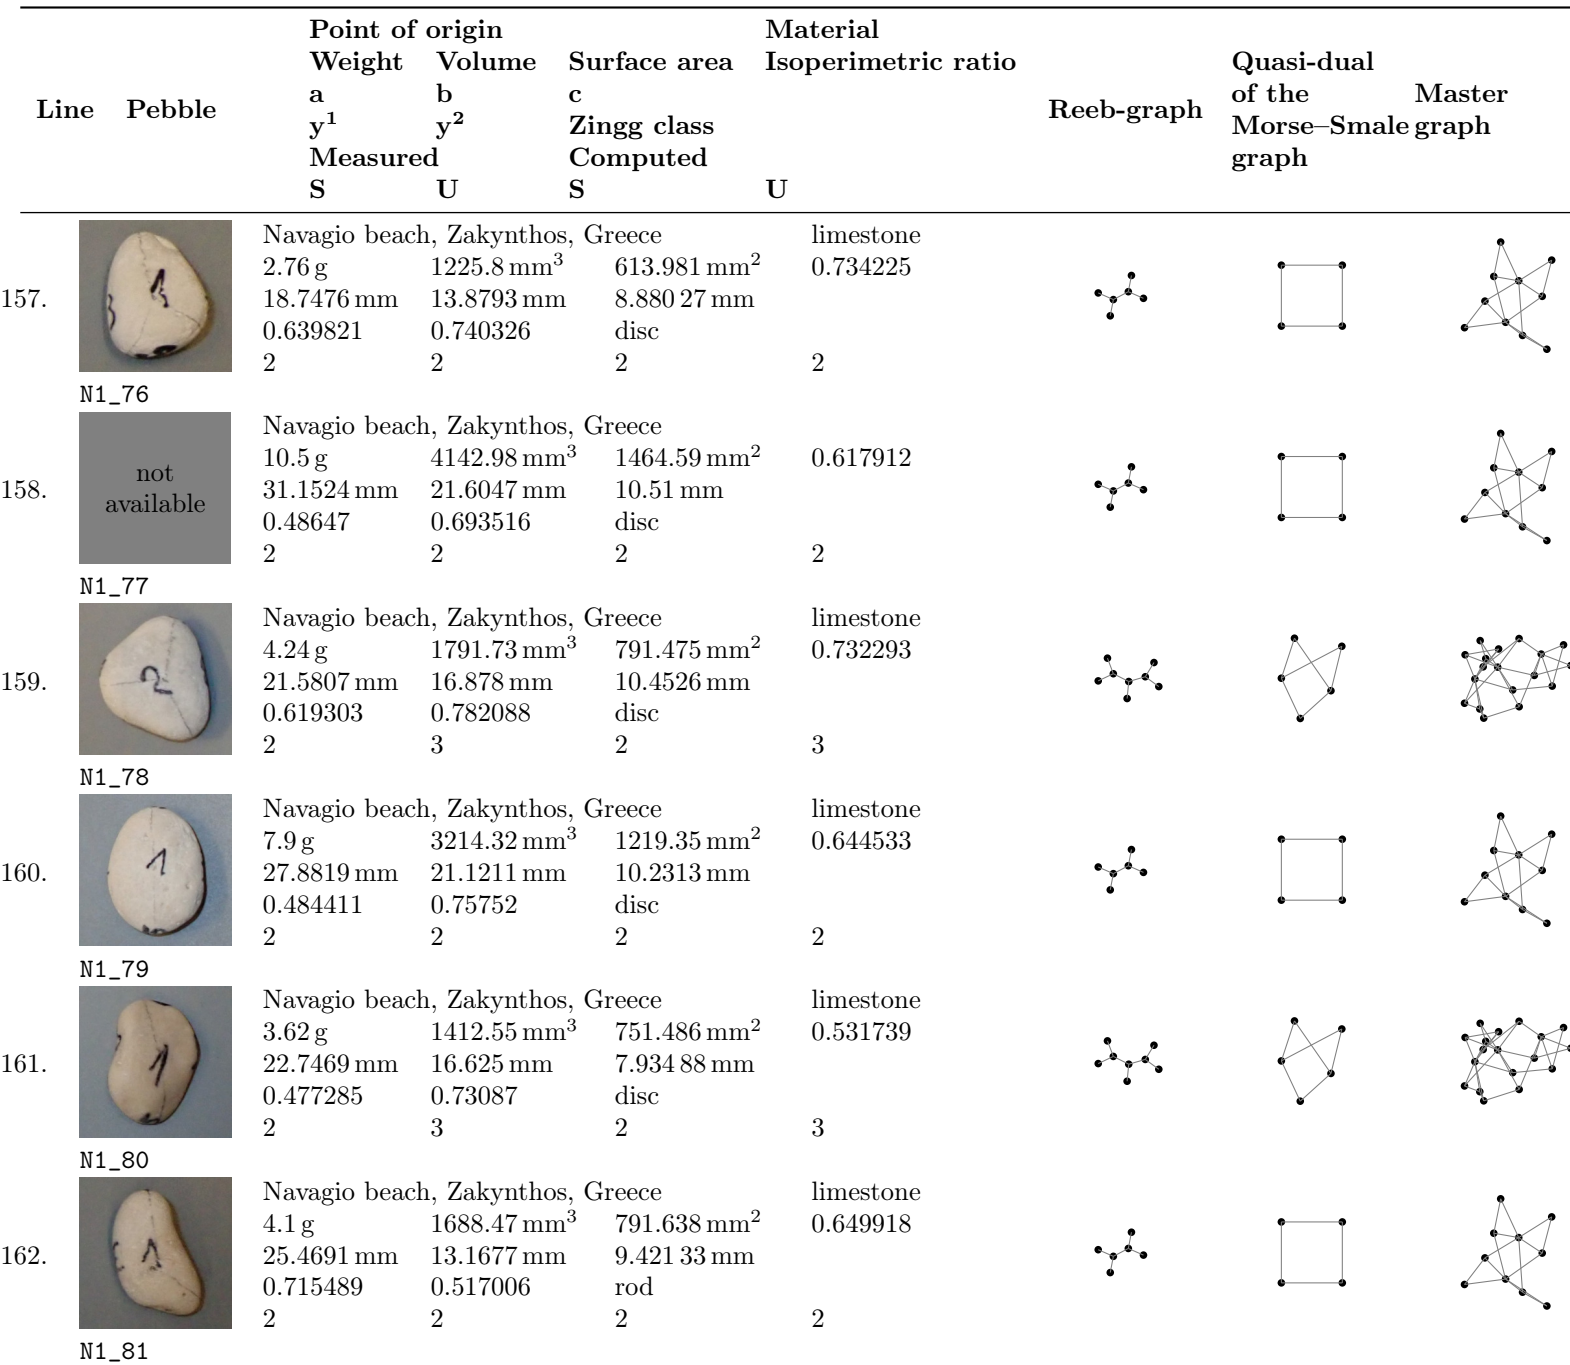 | 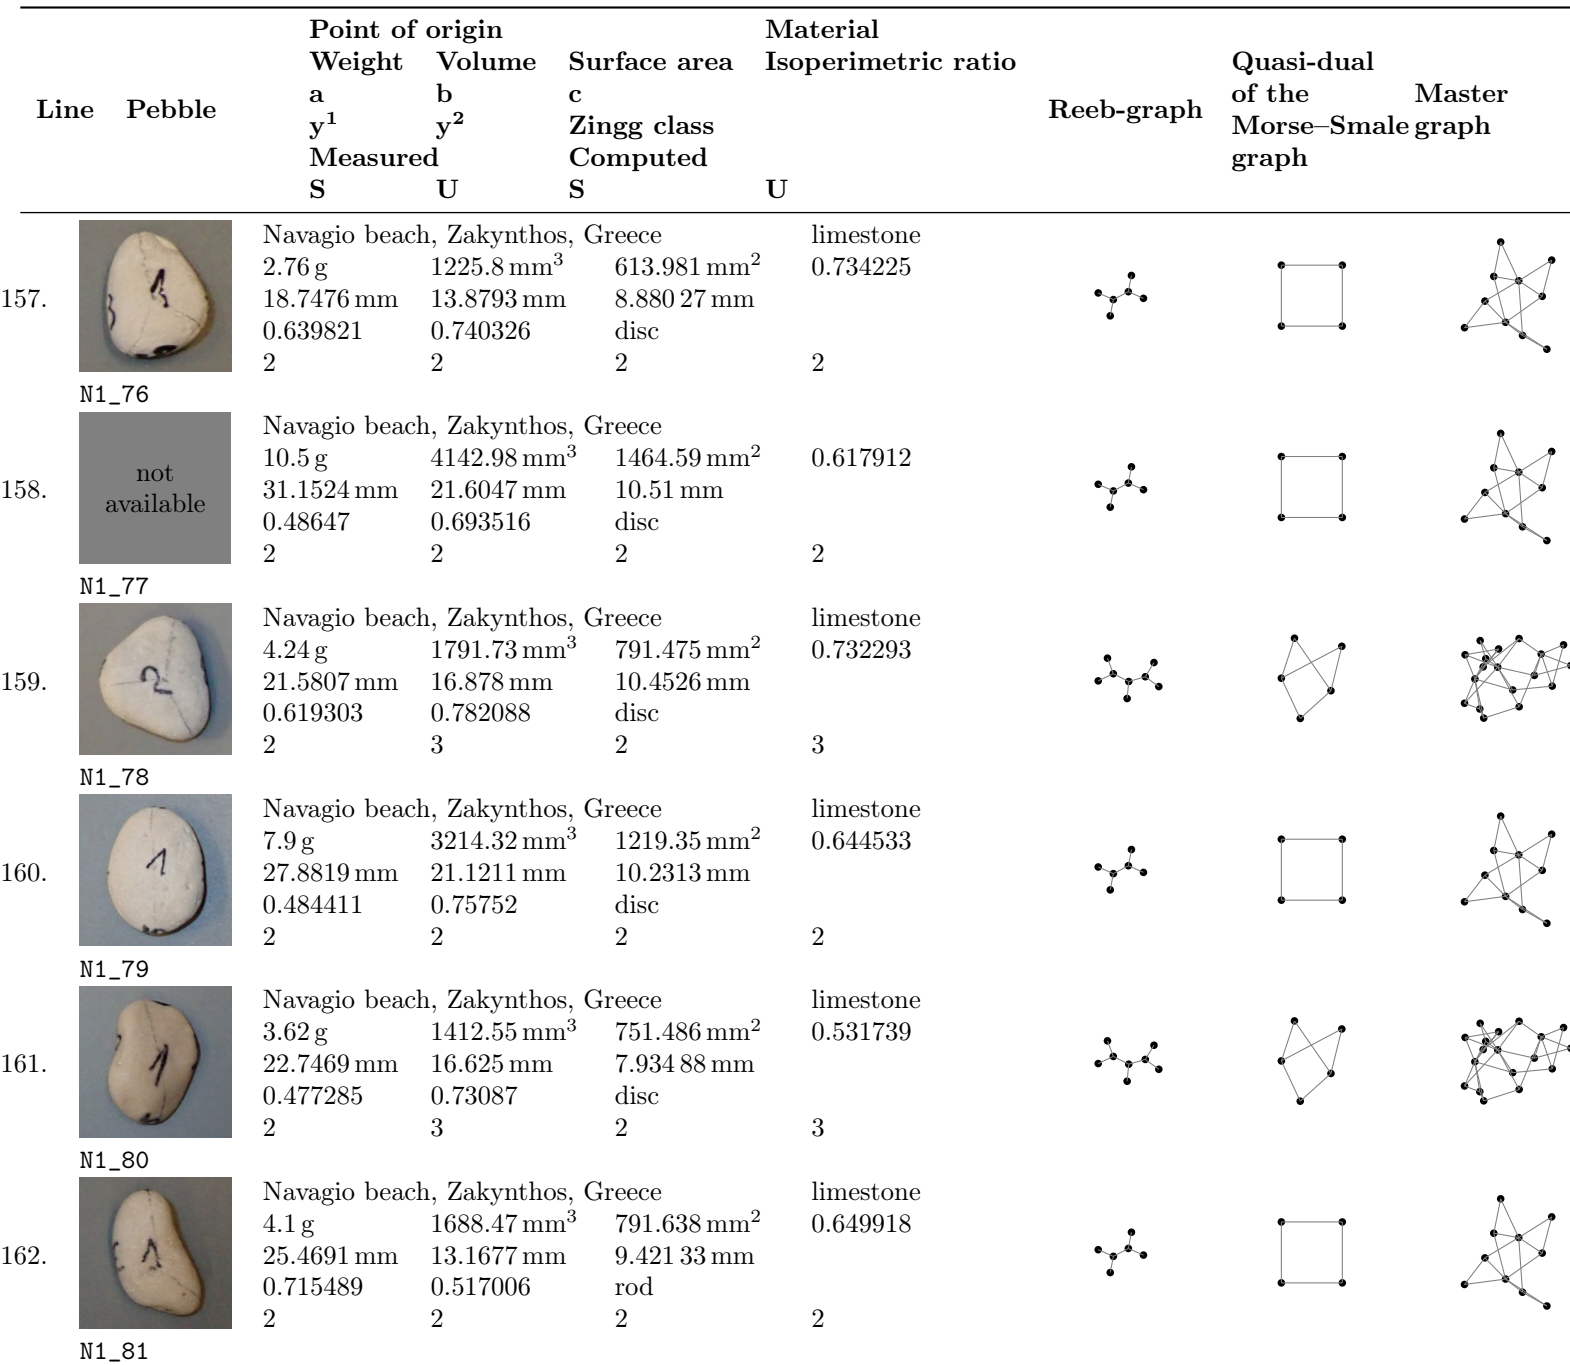 |
|      | N1_81                                                                               |                                                                           |                                                        |                                                     |                                |                     |                                                                                       |                                                                                       |                                                                                       |

| Line | Pebble                                                                              | Point of origin                  |                          |                              | Material              | Reeb-graph                                                                            | Quasi-dual<br>of the<br>Morse–Smale<br>graph                                          | Master<br>graph                                                                       |
|------|-------------------------------------------------------------------------------------|----------------------------------|--------------------------|------------------------------|-----------------------|---------------------------------------------------------------------------------------|---------------------------------------------------------------------------------------|---------------------------------------------------------------------------------------|
|      |                                                                                     | Weight                           | Volume                   | Surface area                 |                       |                                                                                       |                                                                                       |                                                                                       |
|      |                                                                                     | a                                | b                        | c                            |                       |                                                                                       |                                                                                       |                                                                                       |
|      |                                                                                     | y <sup>1</sup><br>Measured<br>S  | y <sup>2</sup><br>U      | Zingg class<br>Computed<br>S |                       |                                                                                       |                                                                                       |                                                                                       |
|      |                                                                                     |                                  |                          |                              | U                     |                                                                                       |                                                                                       |                                                                                       |
| 163. | 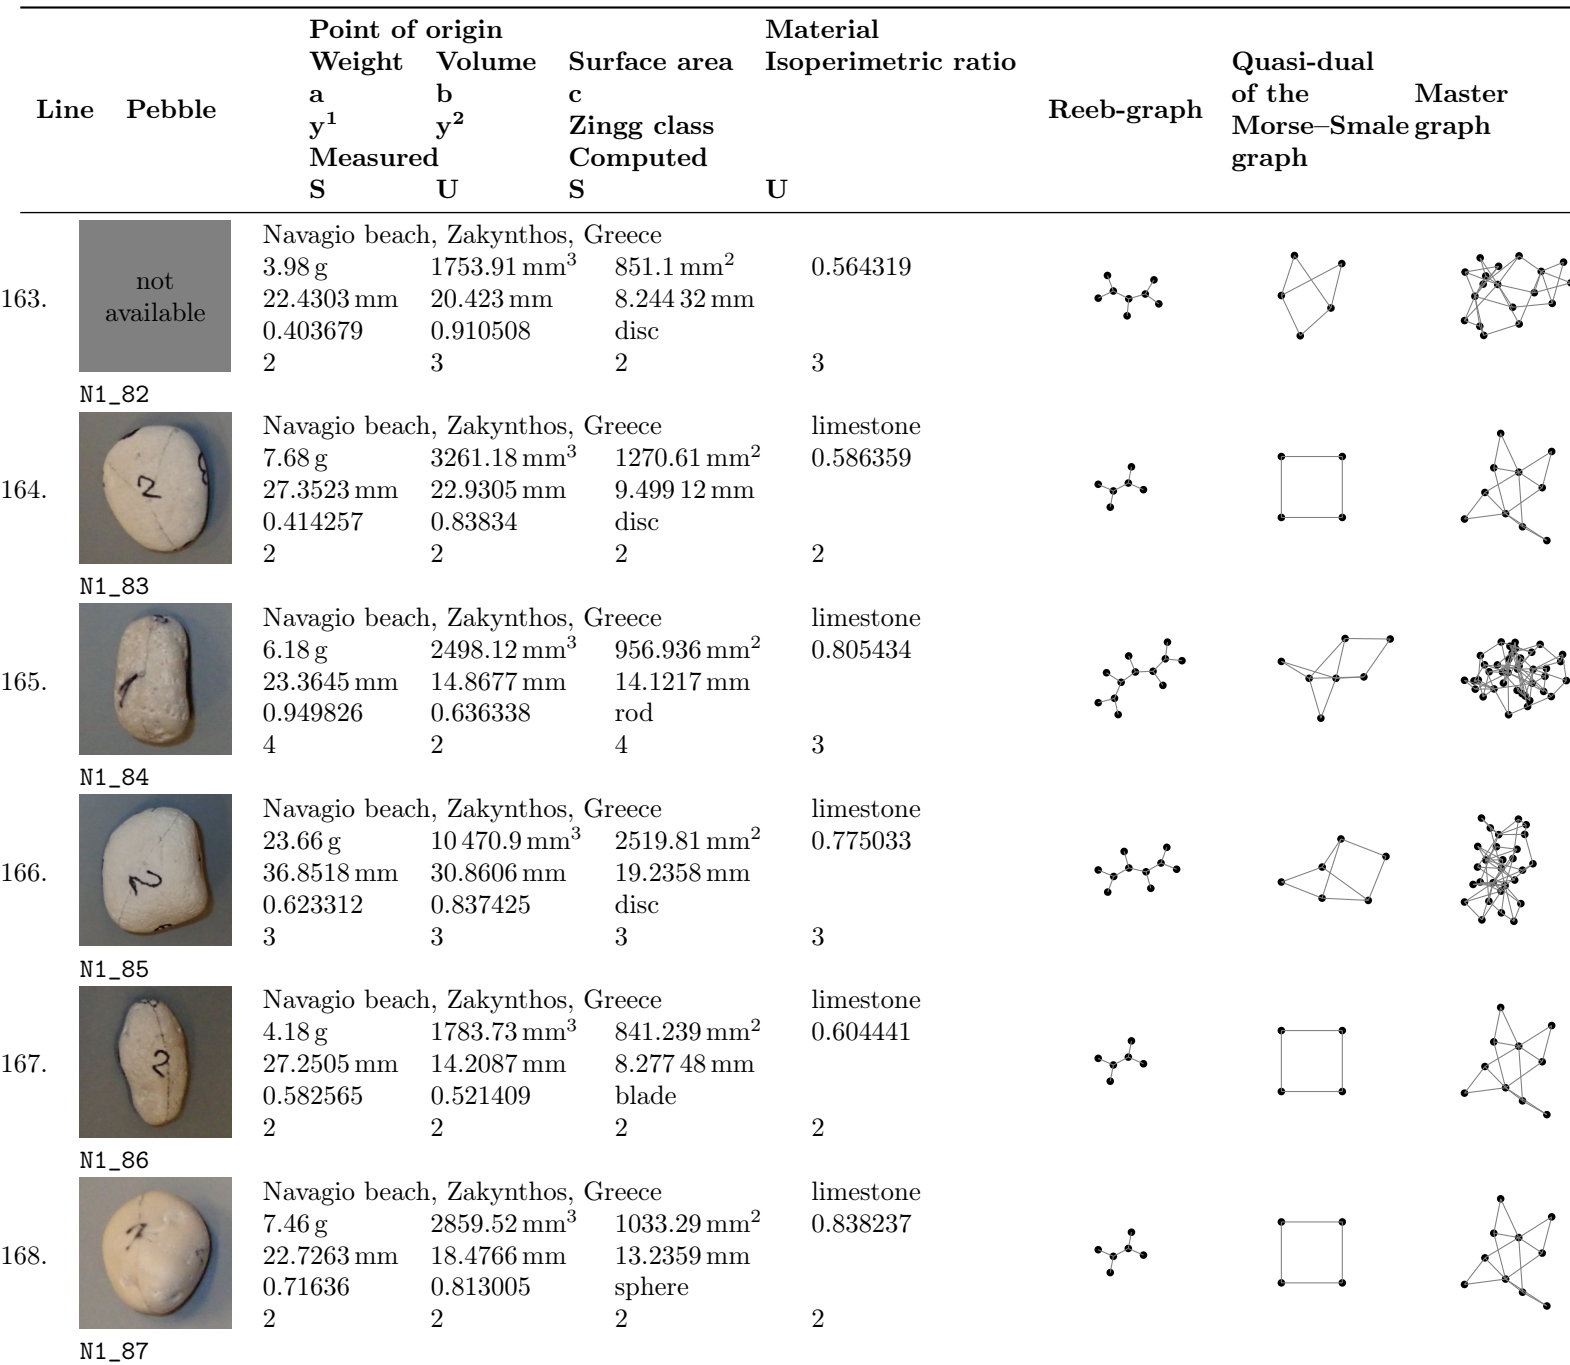   | Navagio beach, Zakynthos, Greece |                          |                              | 0.564319              | 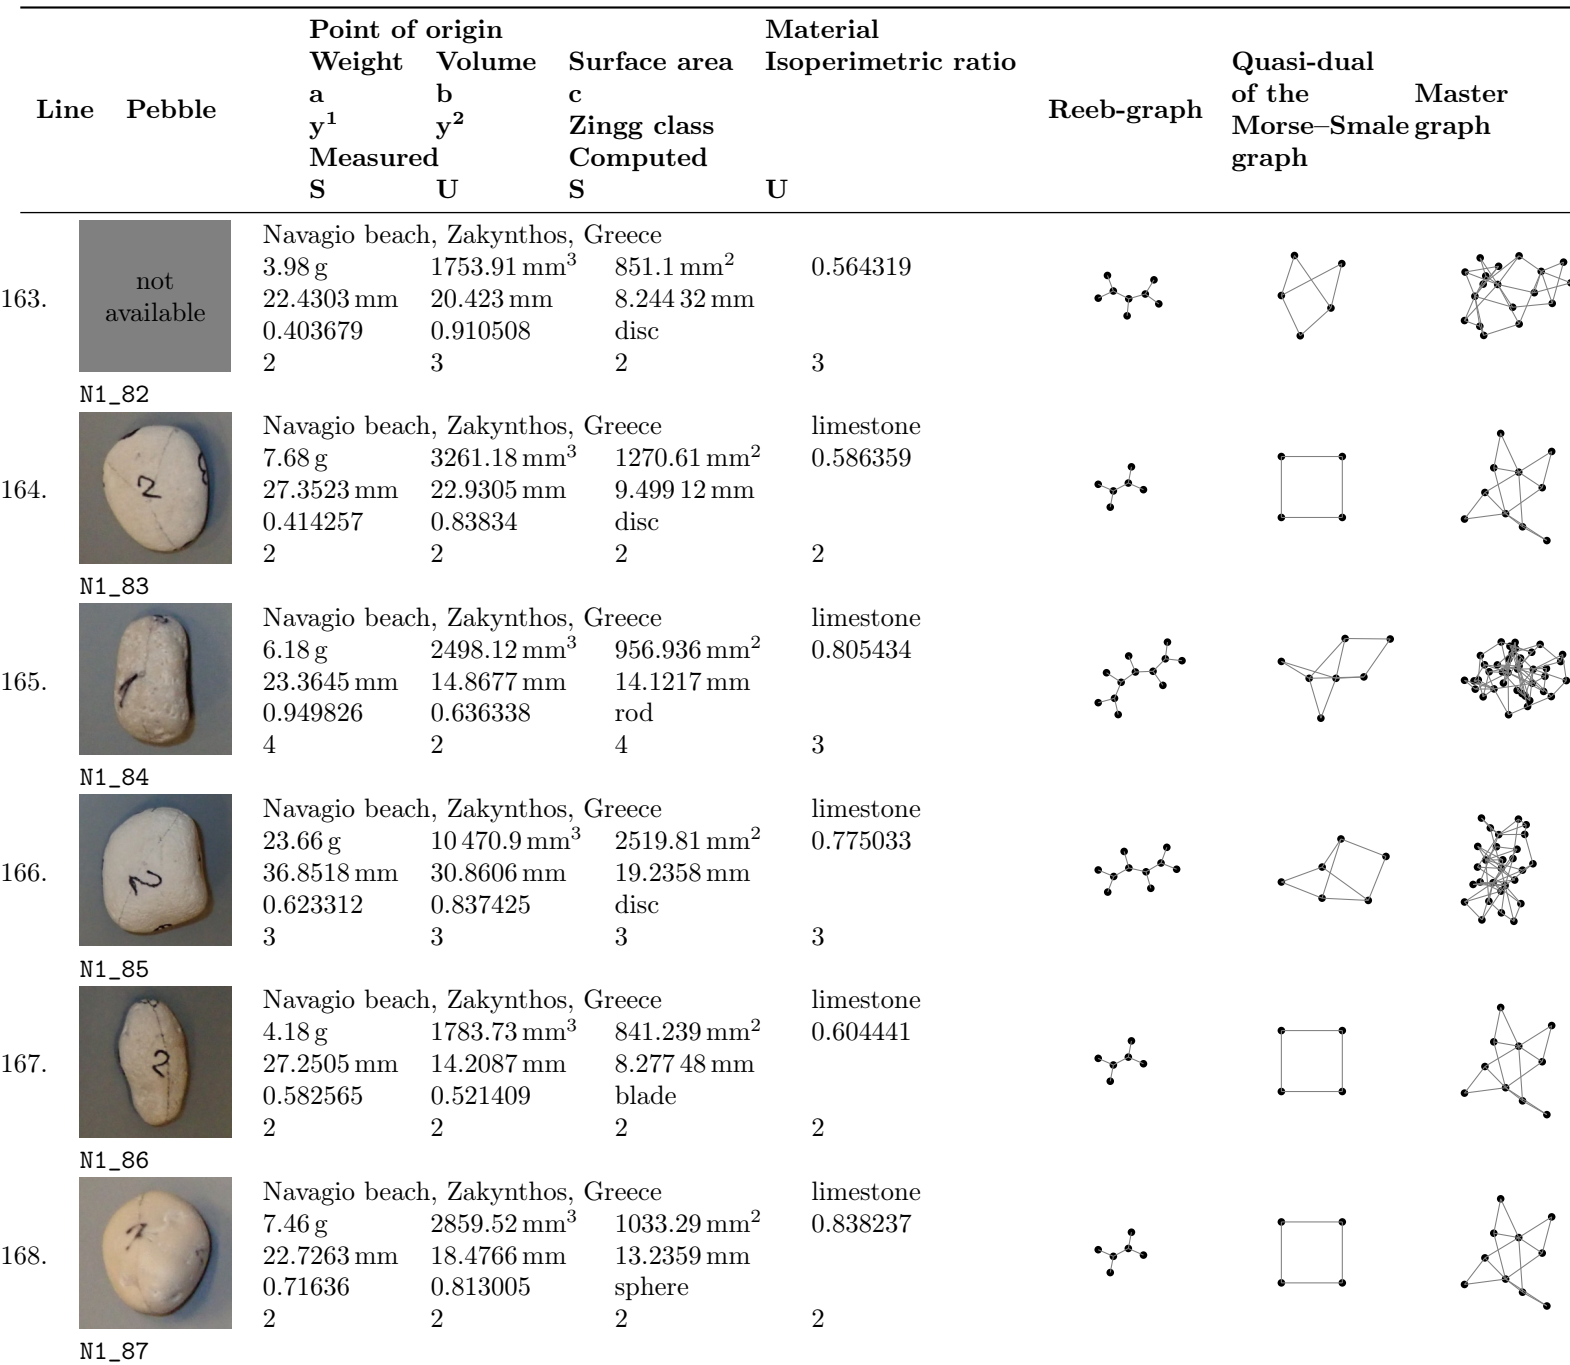   | 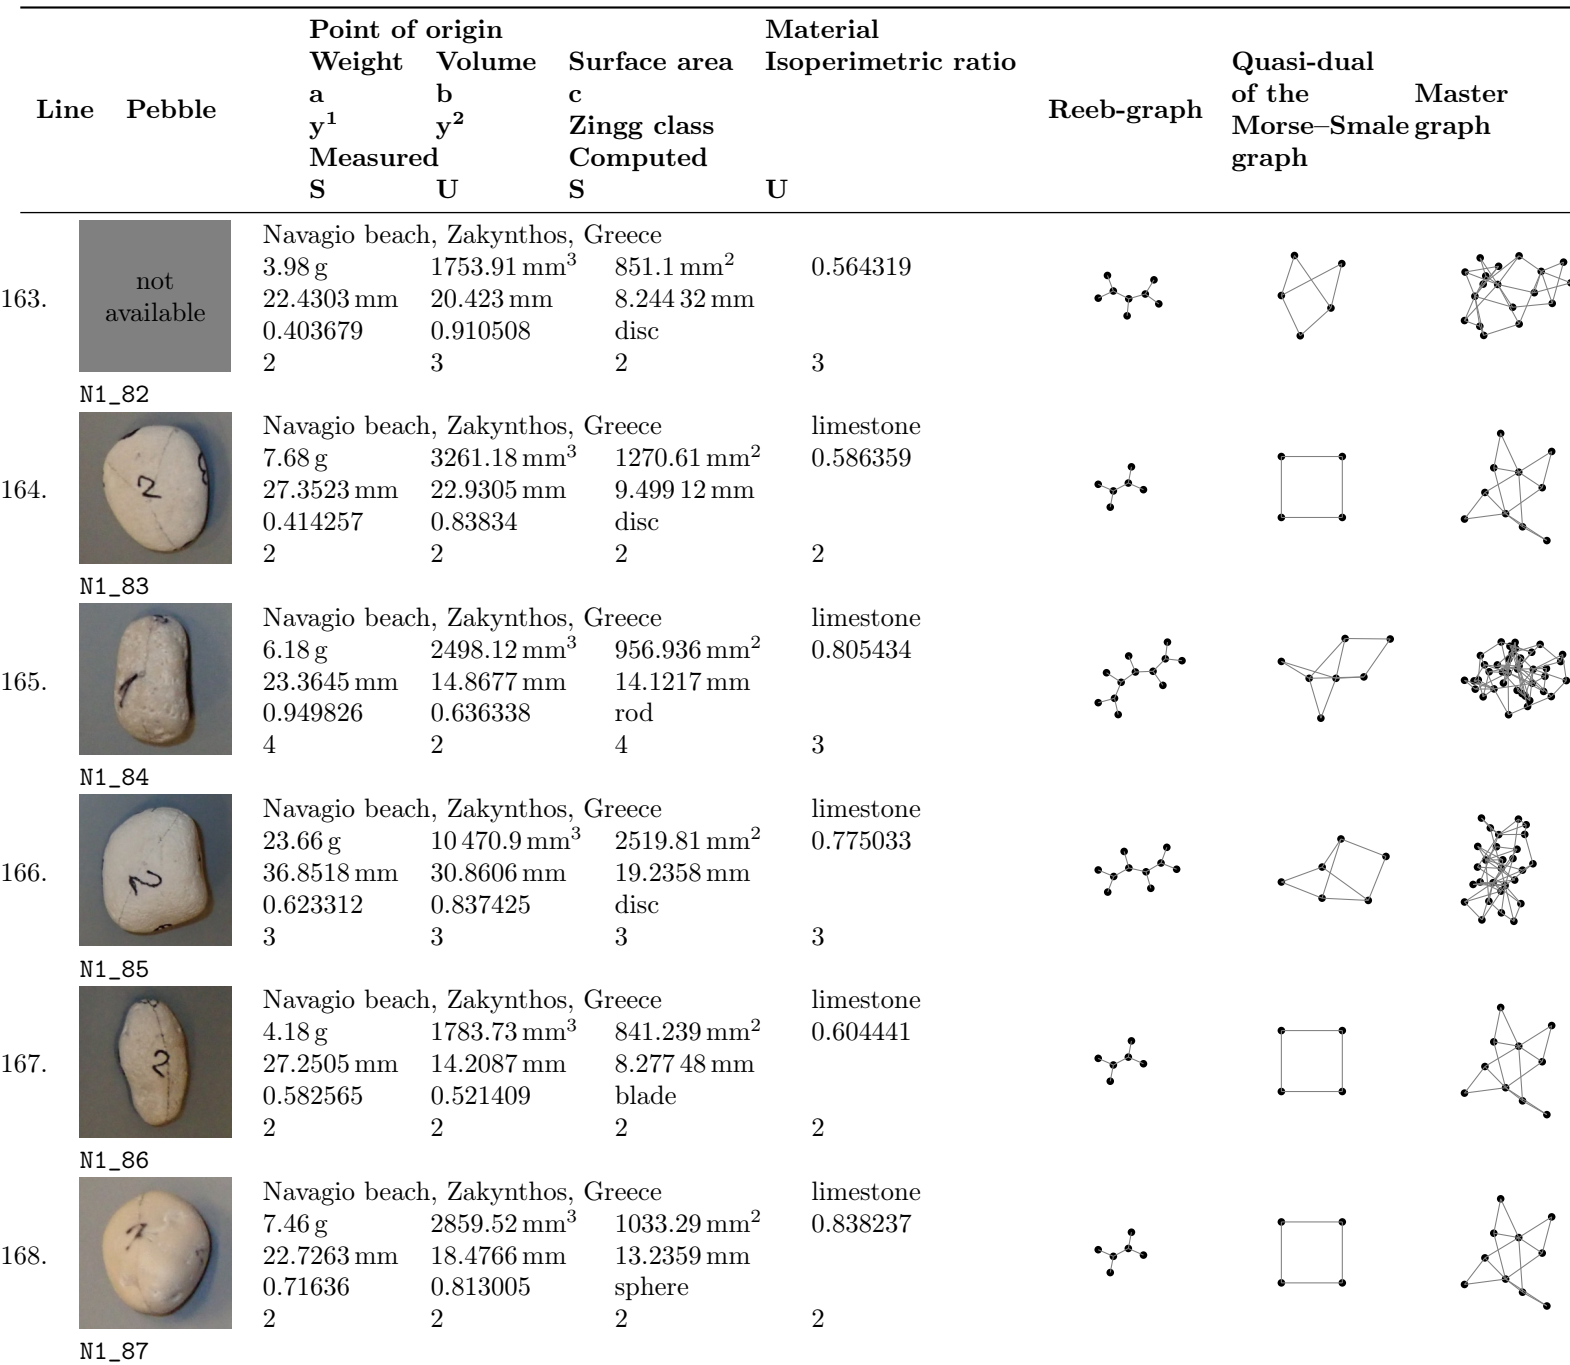   | 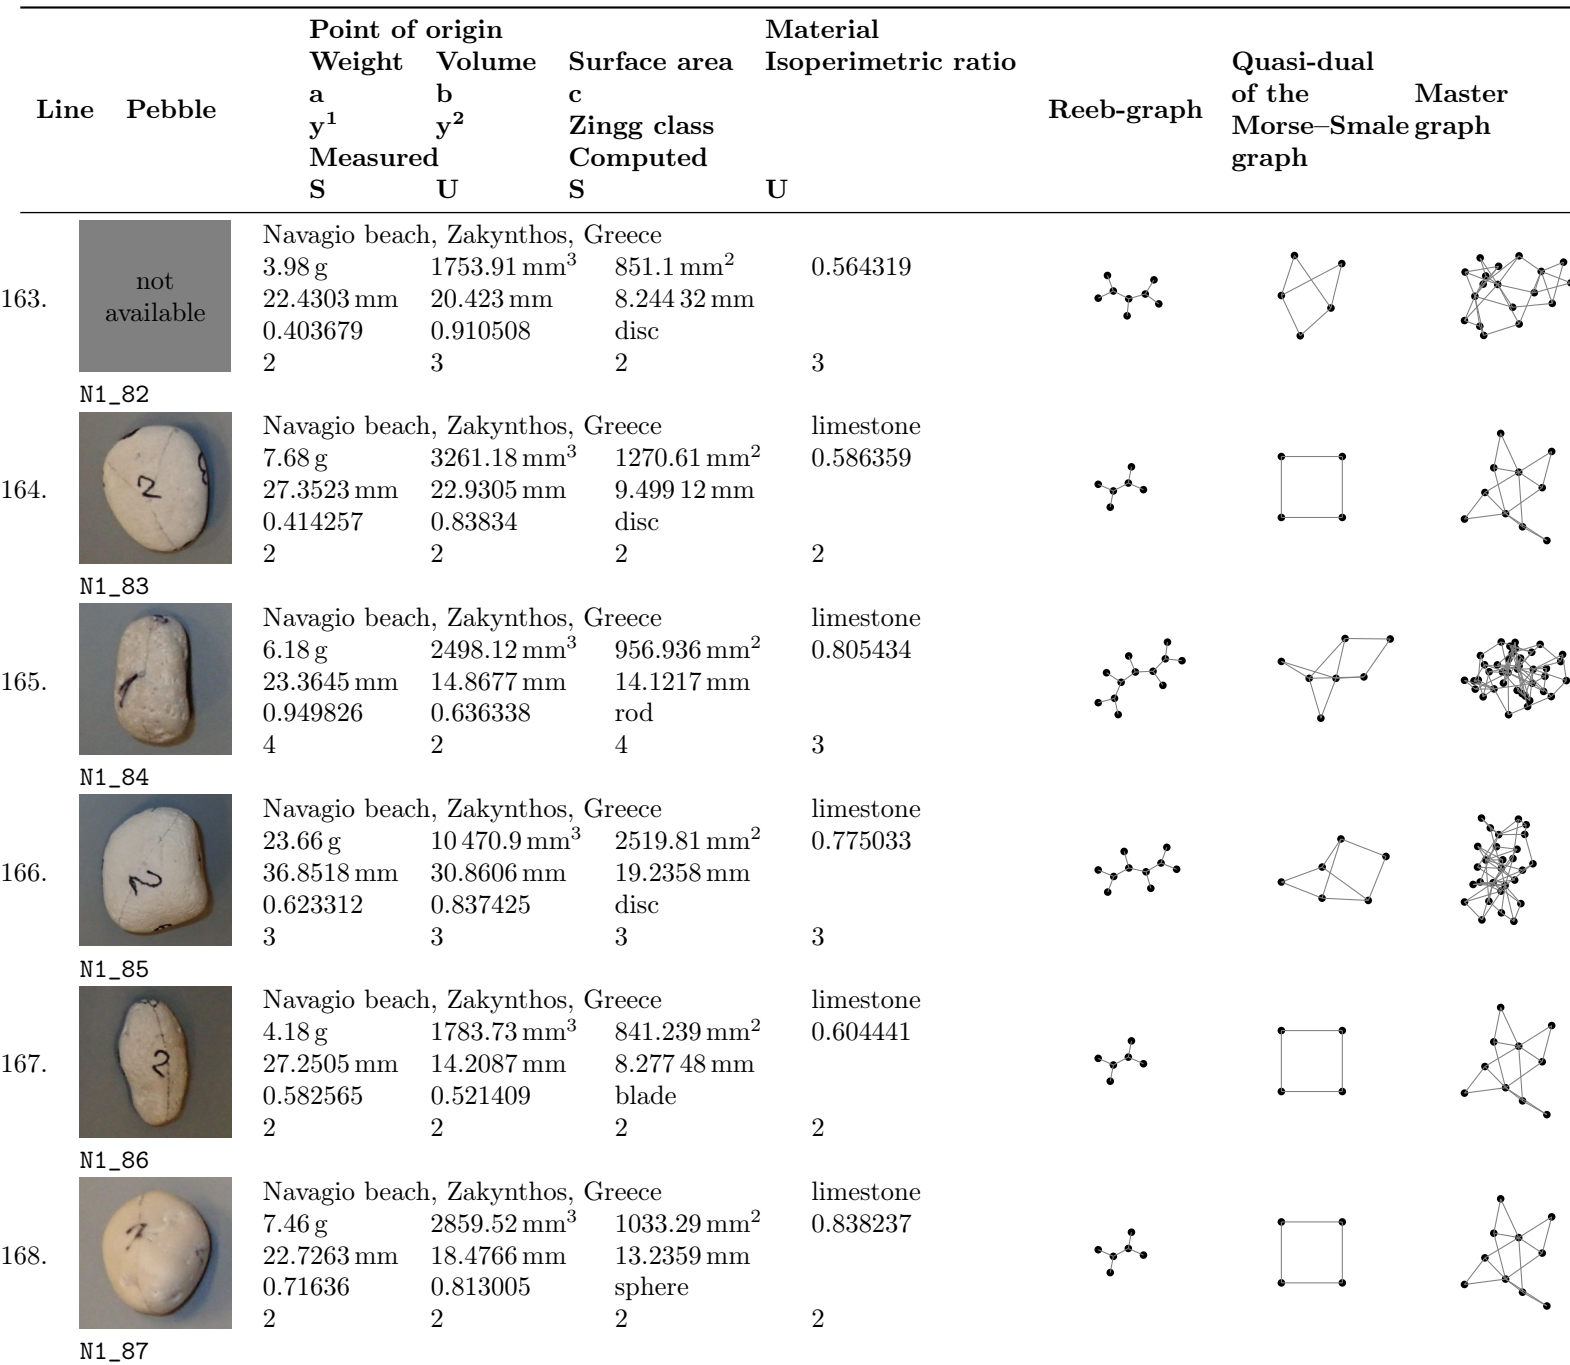   |
|      |                                                                                     | 3.98 g                           | 1753.91 mm <sup>3</sup>  | 851.1 mm <sup>2</sup>        |                       |                                                                                       |                                                                                       |                                                                                       |
|      |                                                                                     | 22.4303 mm                       | 20.423 mm                | 8.244 32 mm                  |                       |                                                                                       |                                                                                       |                                                                                       |
|      |                                                                                     | 0.403679                         | 0.910508                 | disc                         |                       |                                                                                       |                                                                                       |                                                                                       |
|      |                                                                                     | 2                                | 3                        | 2                            |                       |                                                                                       |                                                                                       |                                                                                       |
|      | N1_82                                                                               |                                  |                          |                              | 3                     |                                                                                       |                                                                                       |                                                                                       |
| 164. | 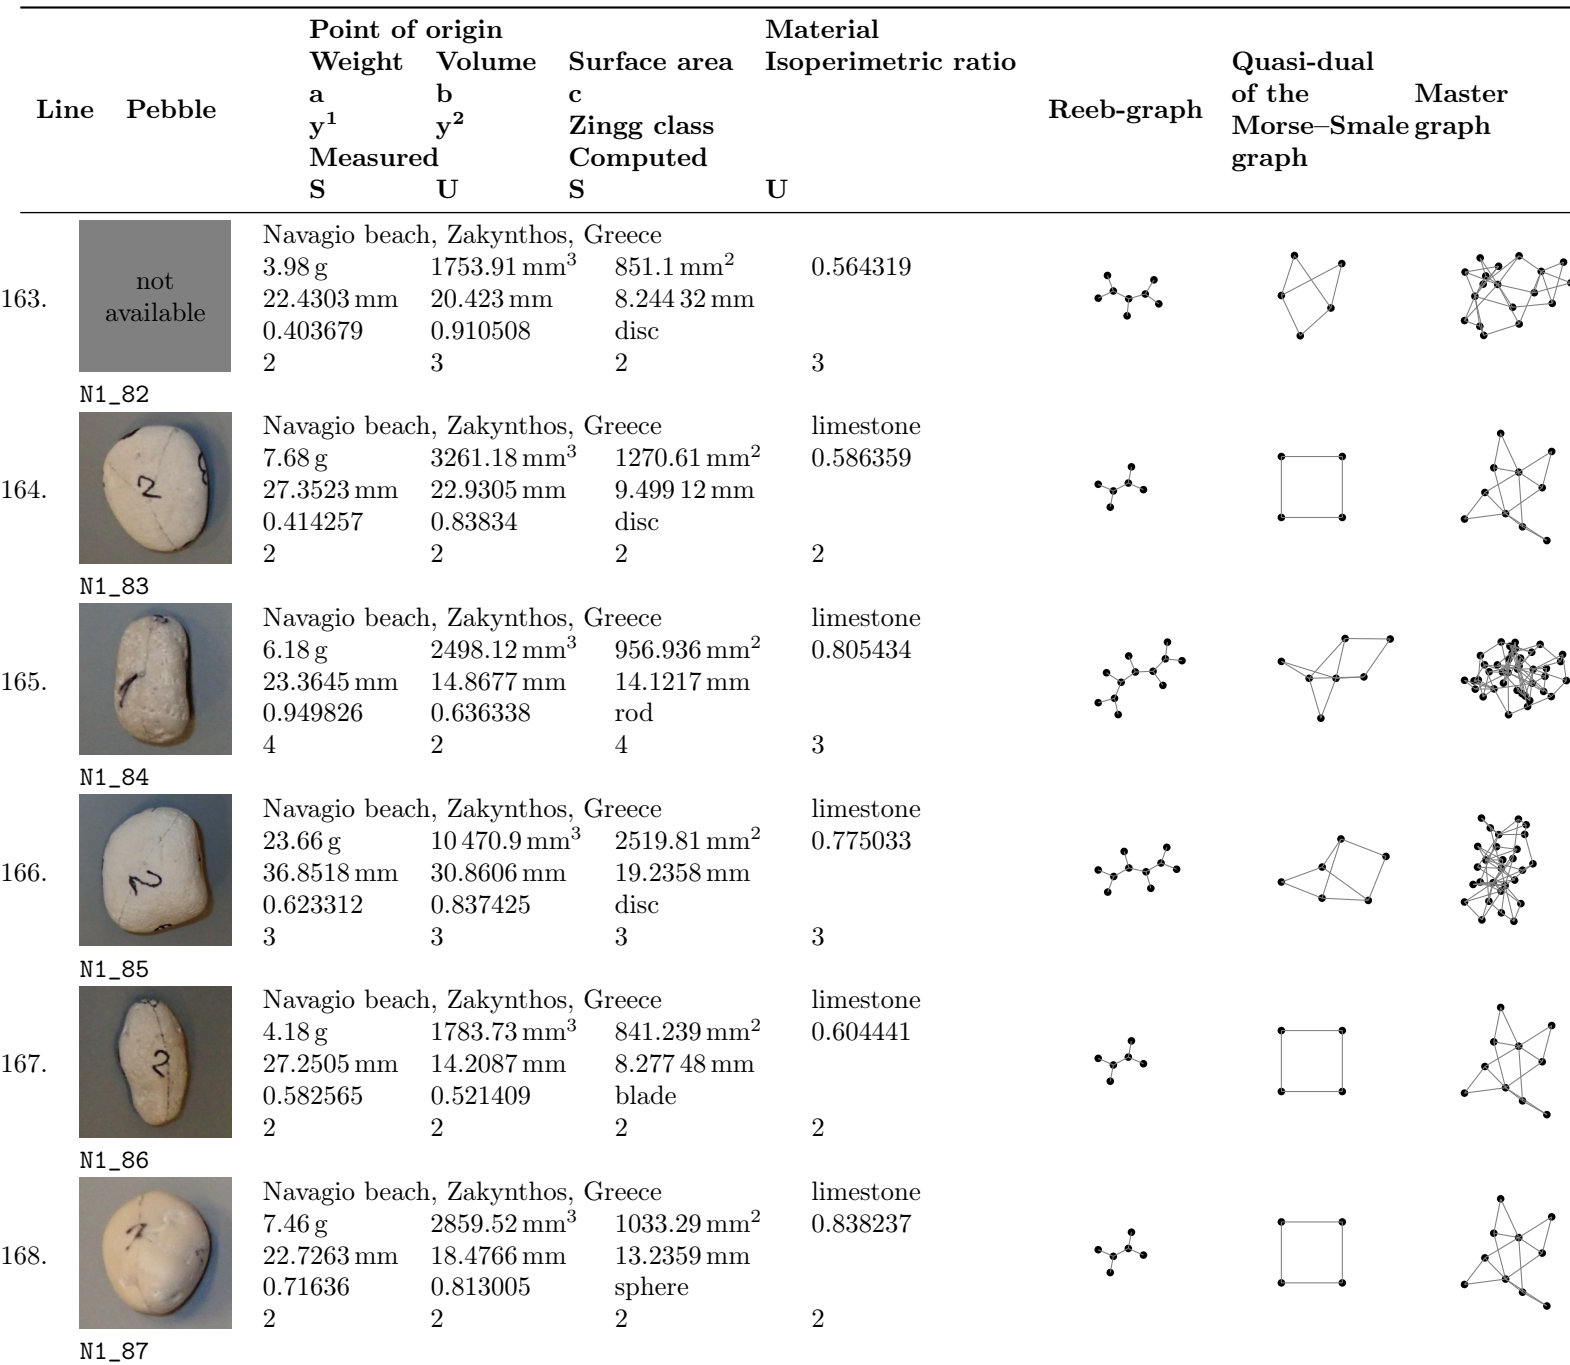   | Navagio beach, Zakynthos, Greece |                          |                              | limestone<br>0.586359 | 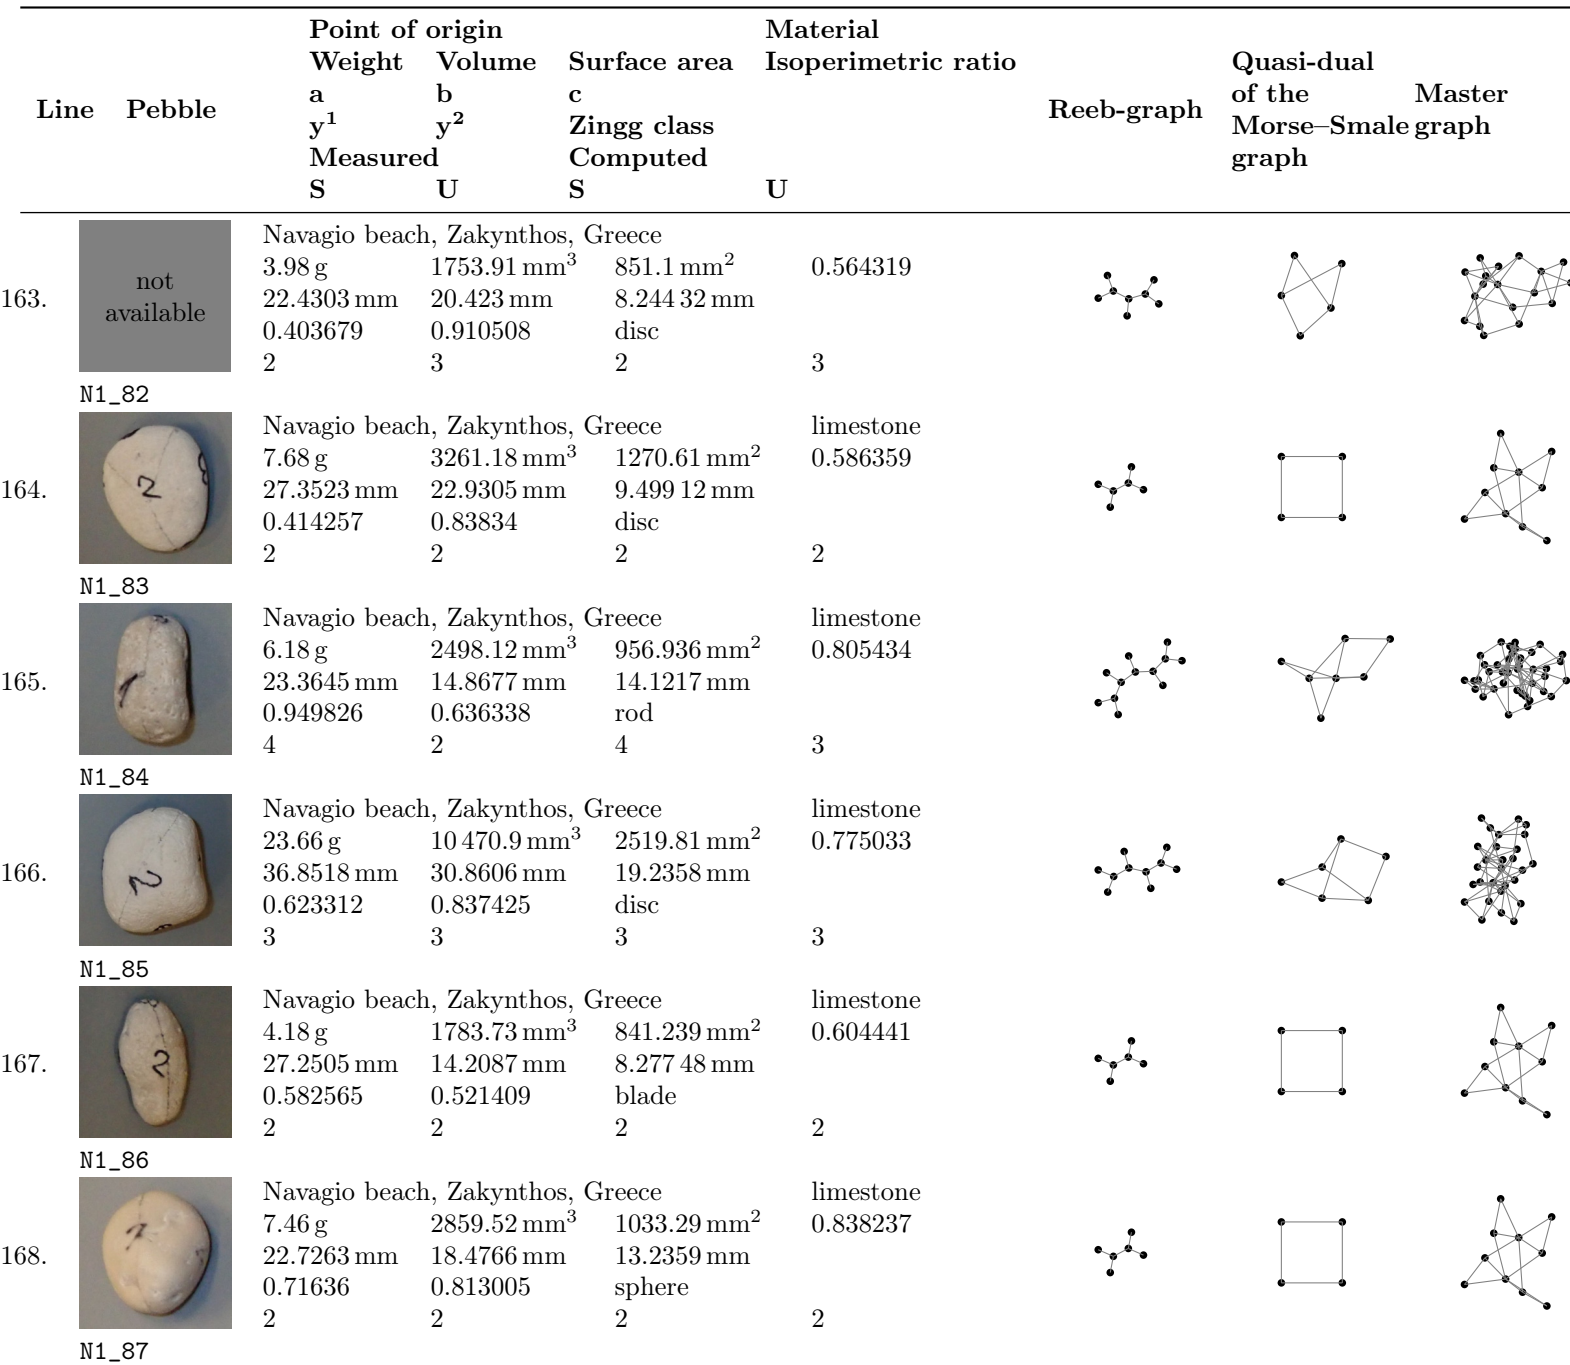   | 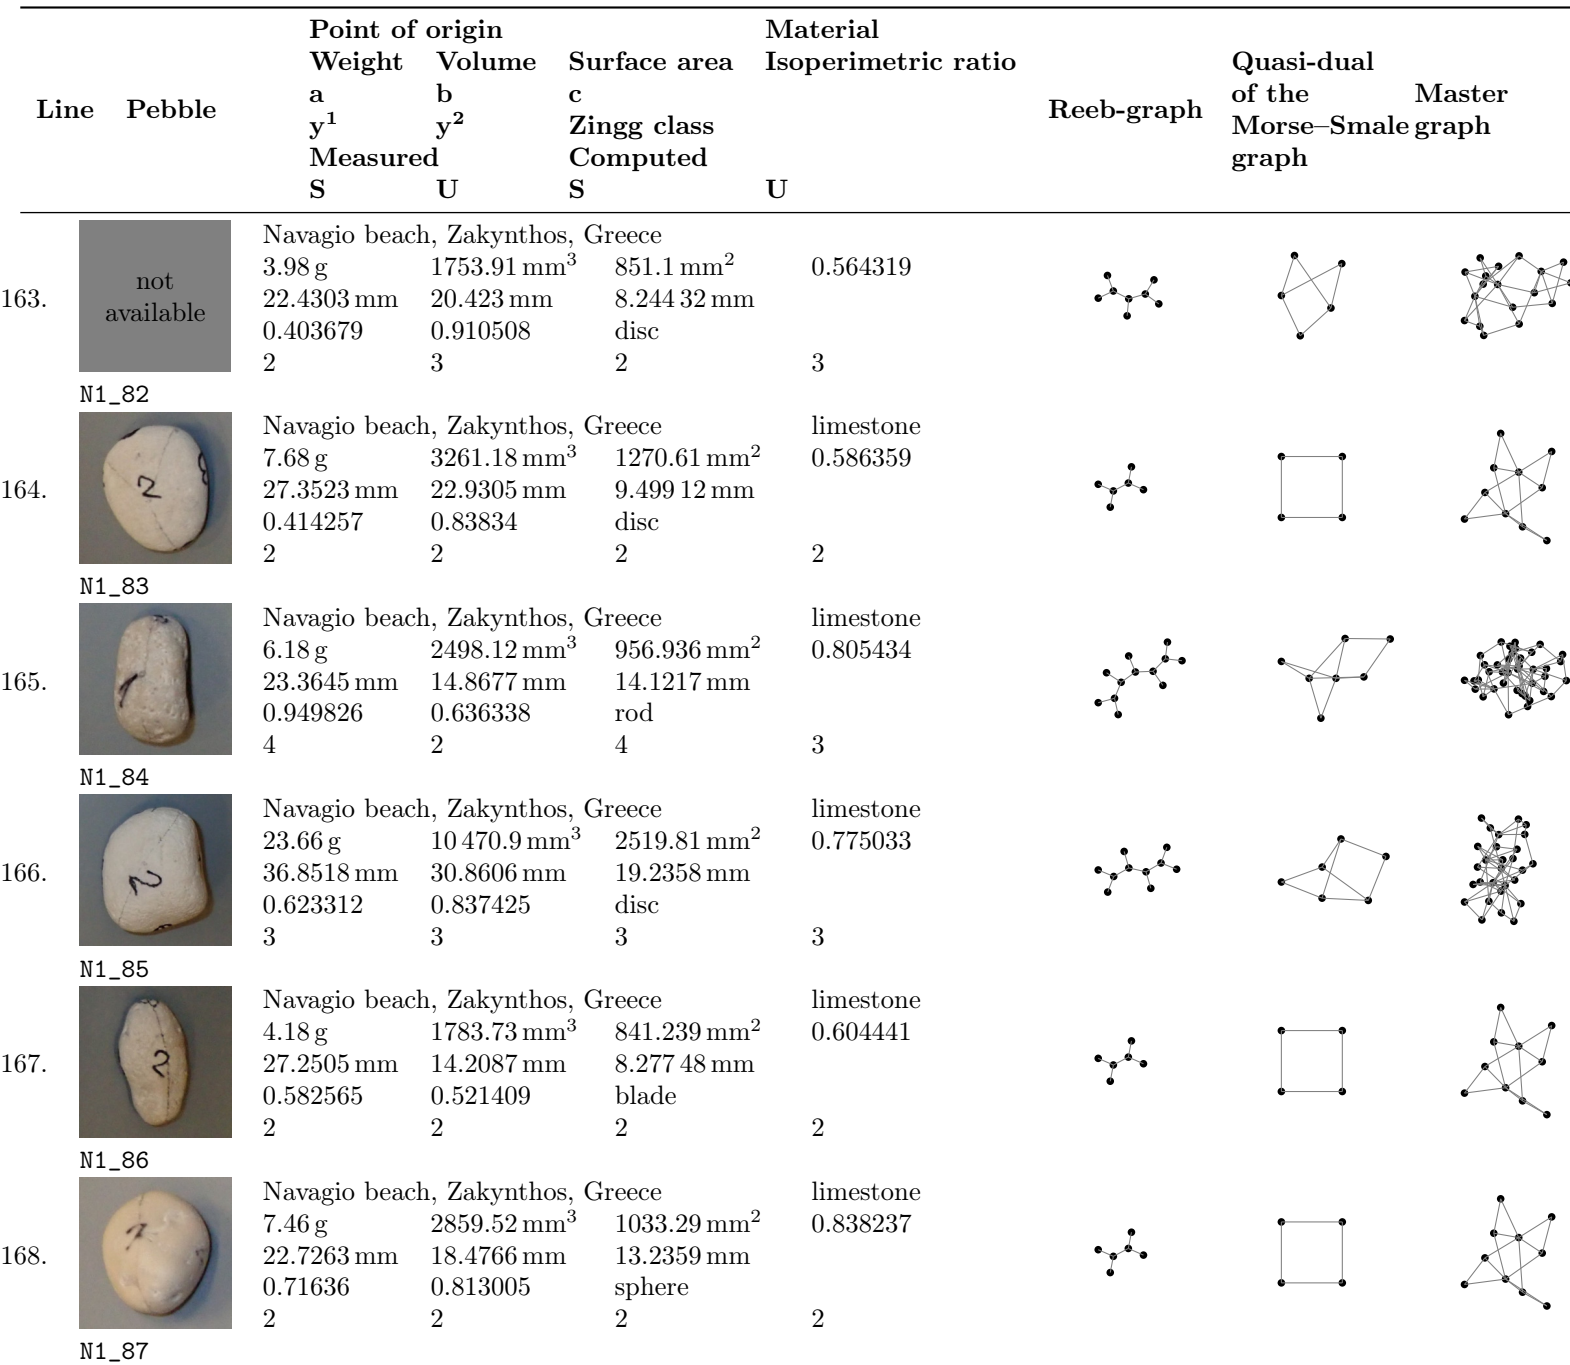   | 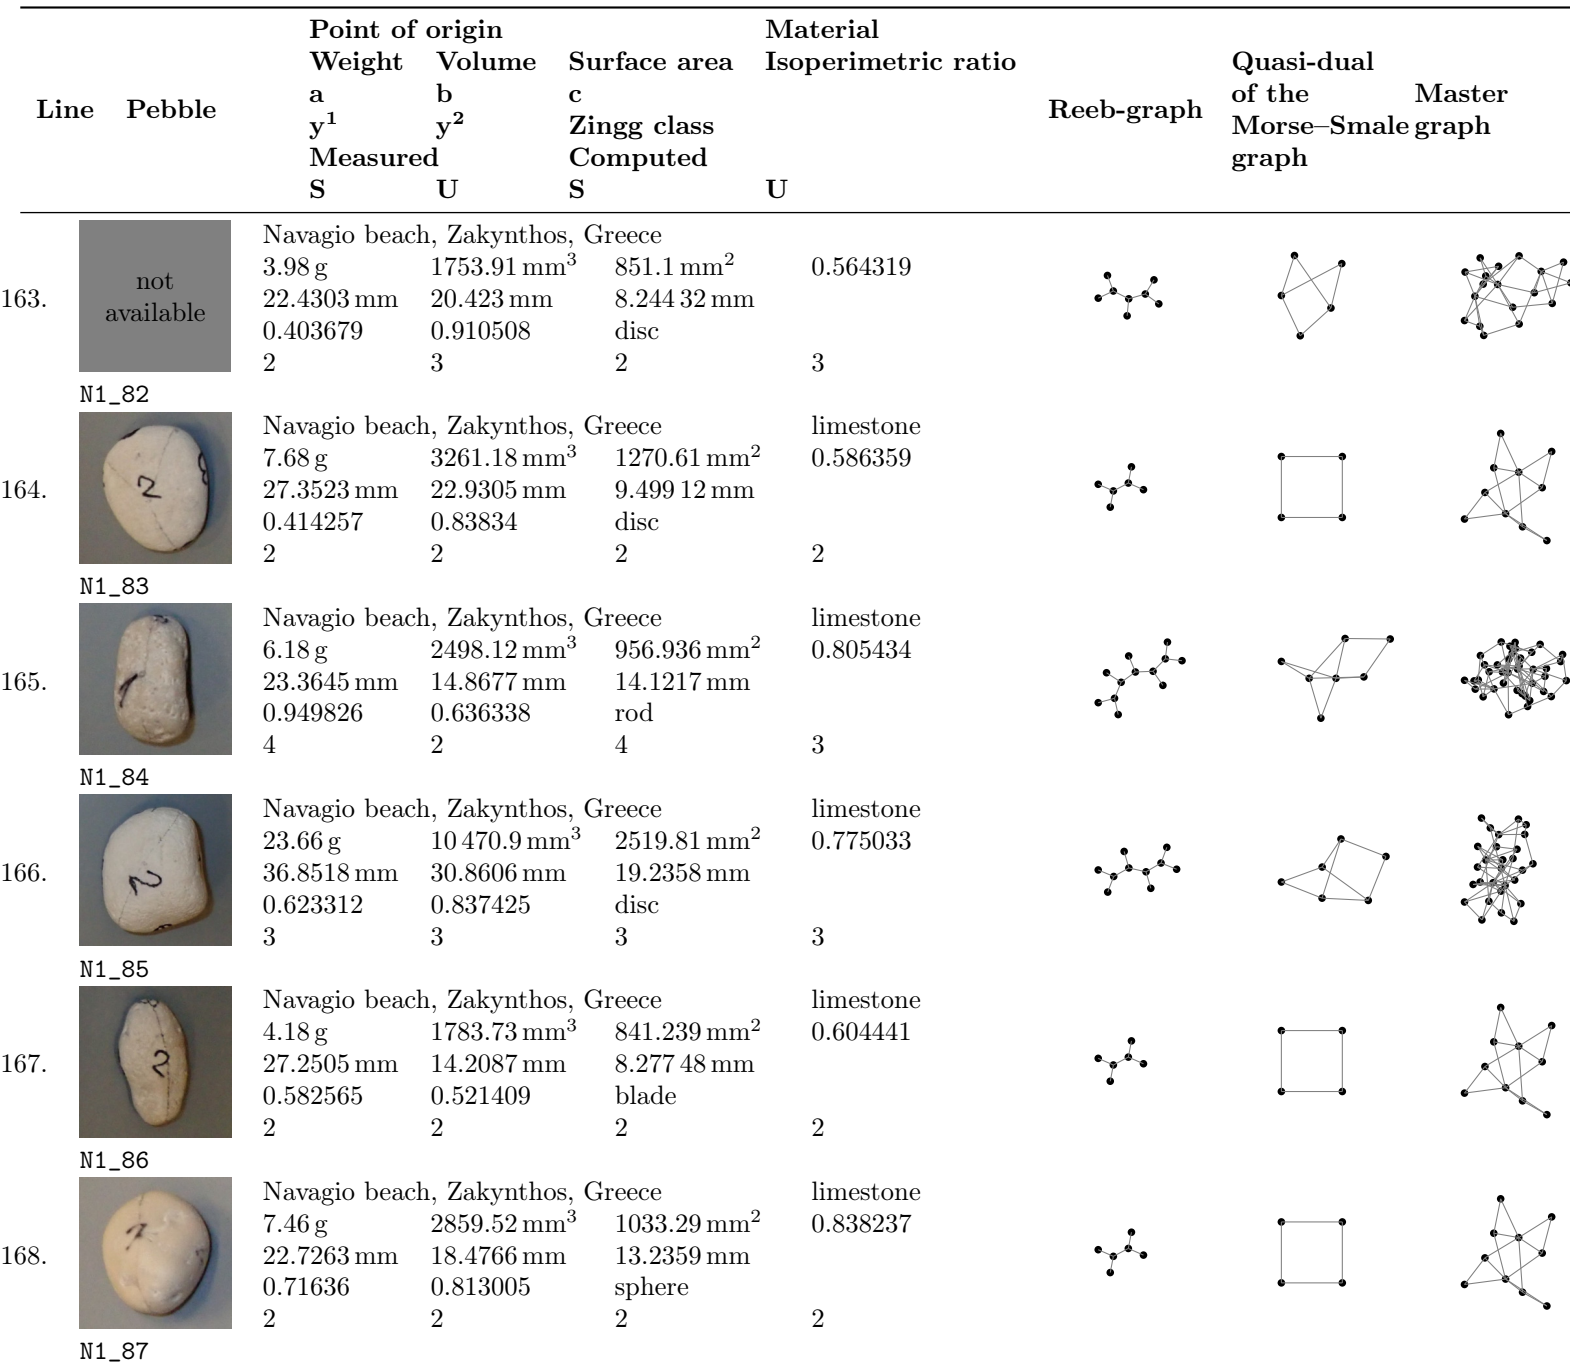   |
|      |                                                                                     | 7.68 g                           | 3261.18 mm <sup>3</sup>  | 1270.61 mm <sup>2</sup>      |                       |                                                                                       |                                                                                       |                                                                                       |
|      |                                                                                     | 27.3523 mm                       | 22.9305 mm               | 9.499 12 mm                  |                       |                                                                                       |                                                                                       |                                                                                       |
|      |                                                                                     | 0.414257                         | 0.83834                  | disc                         |                       |                                                                                       |                                                                                       |                                                                                       |
|      |                                                                                     | 2                                | 2                        | 2                            |                       |                                                                                       |                                                                                       |                                                                                       |
|      | N1_83                                                                               |                                  |                          |                              | 2                     |                                                                                       |                                                                                       |                                                                                       |
| 165. | 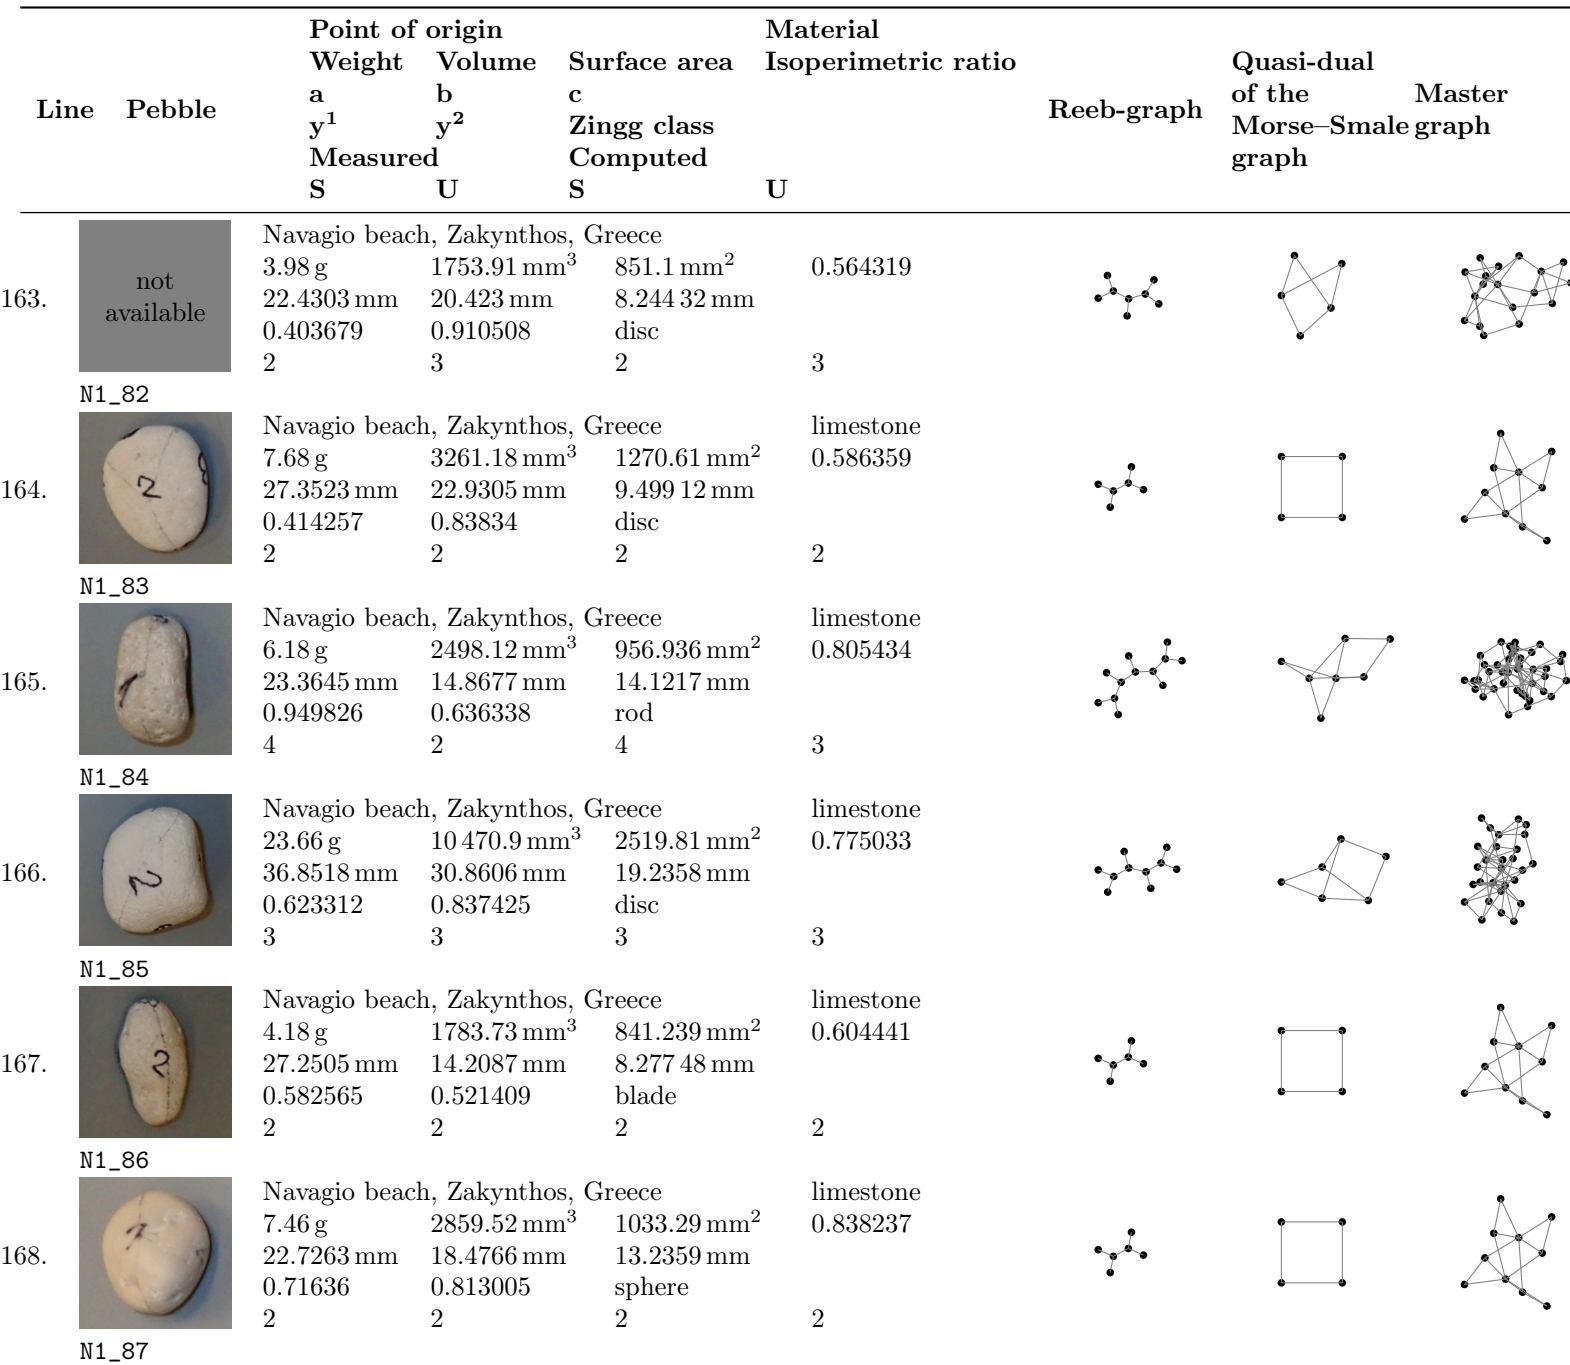   | Navagio beach, Zakynthos, Greece |                          |                              | limestone<br>0.805434 | 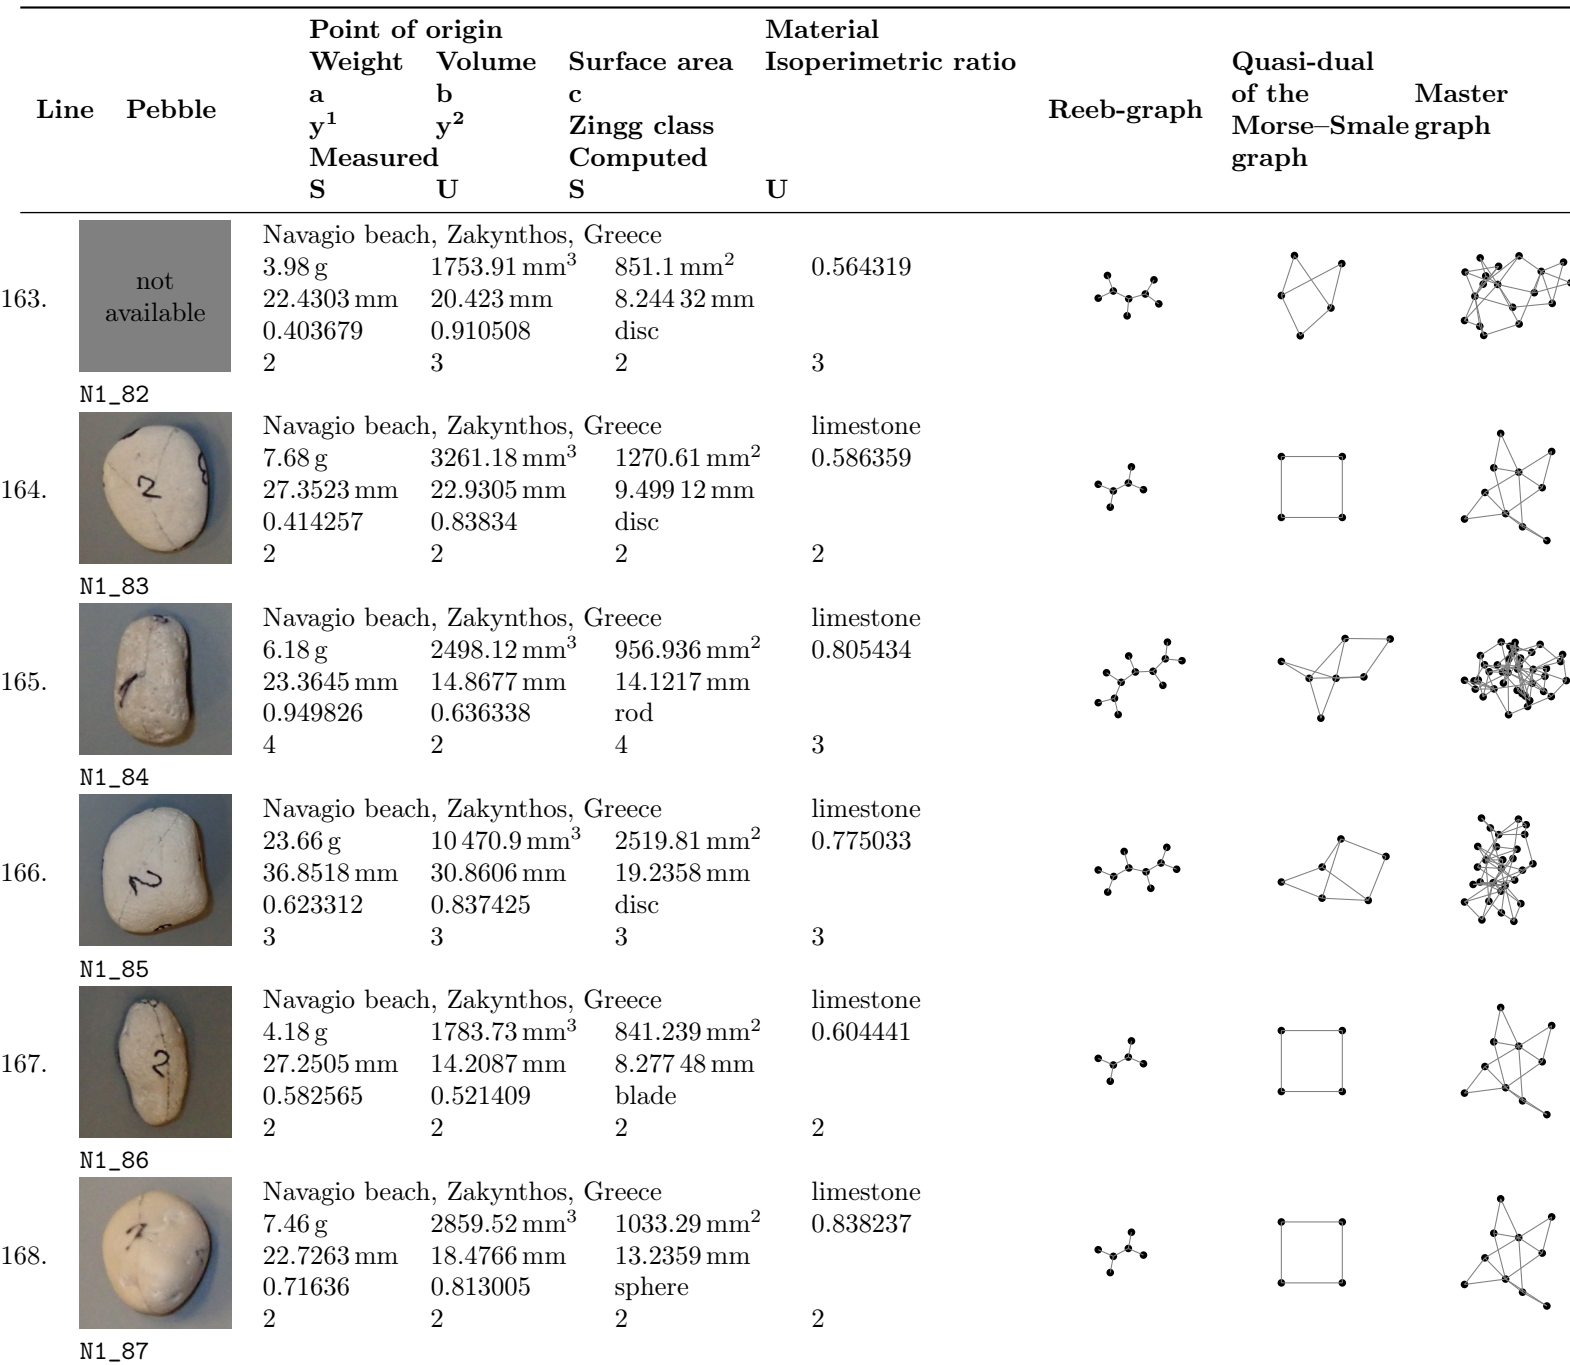   | 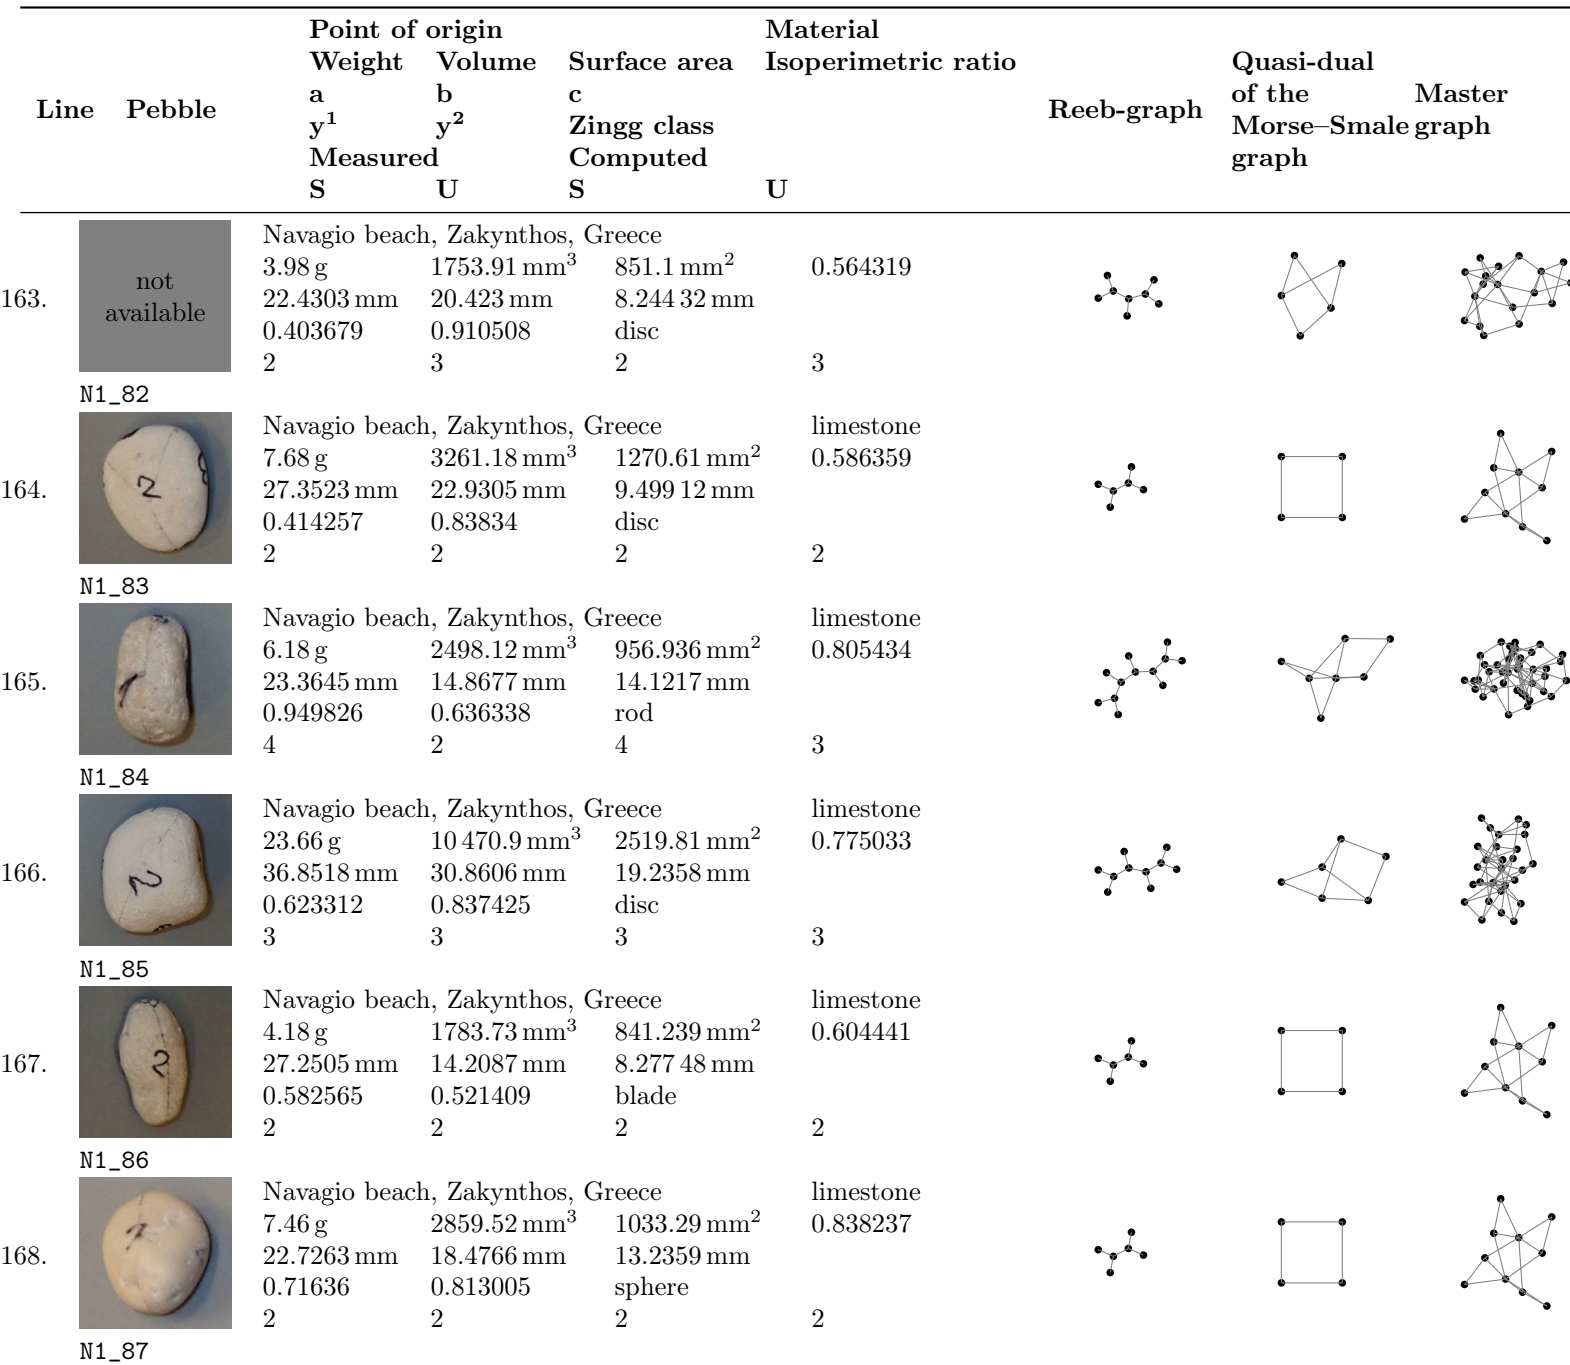   | 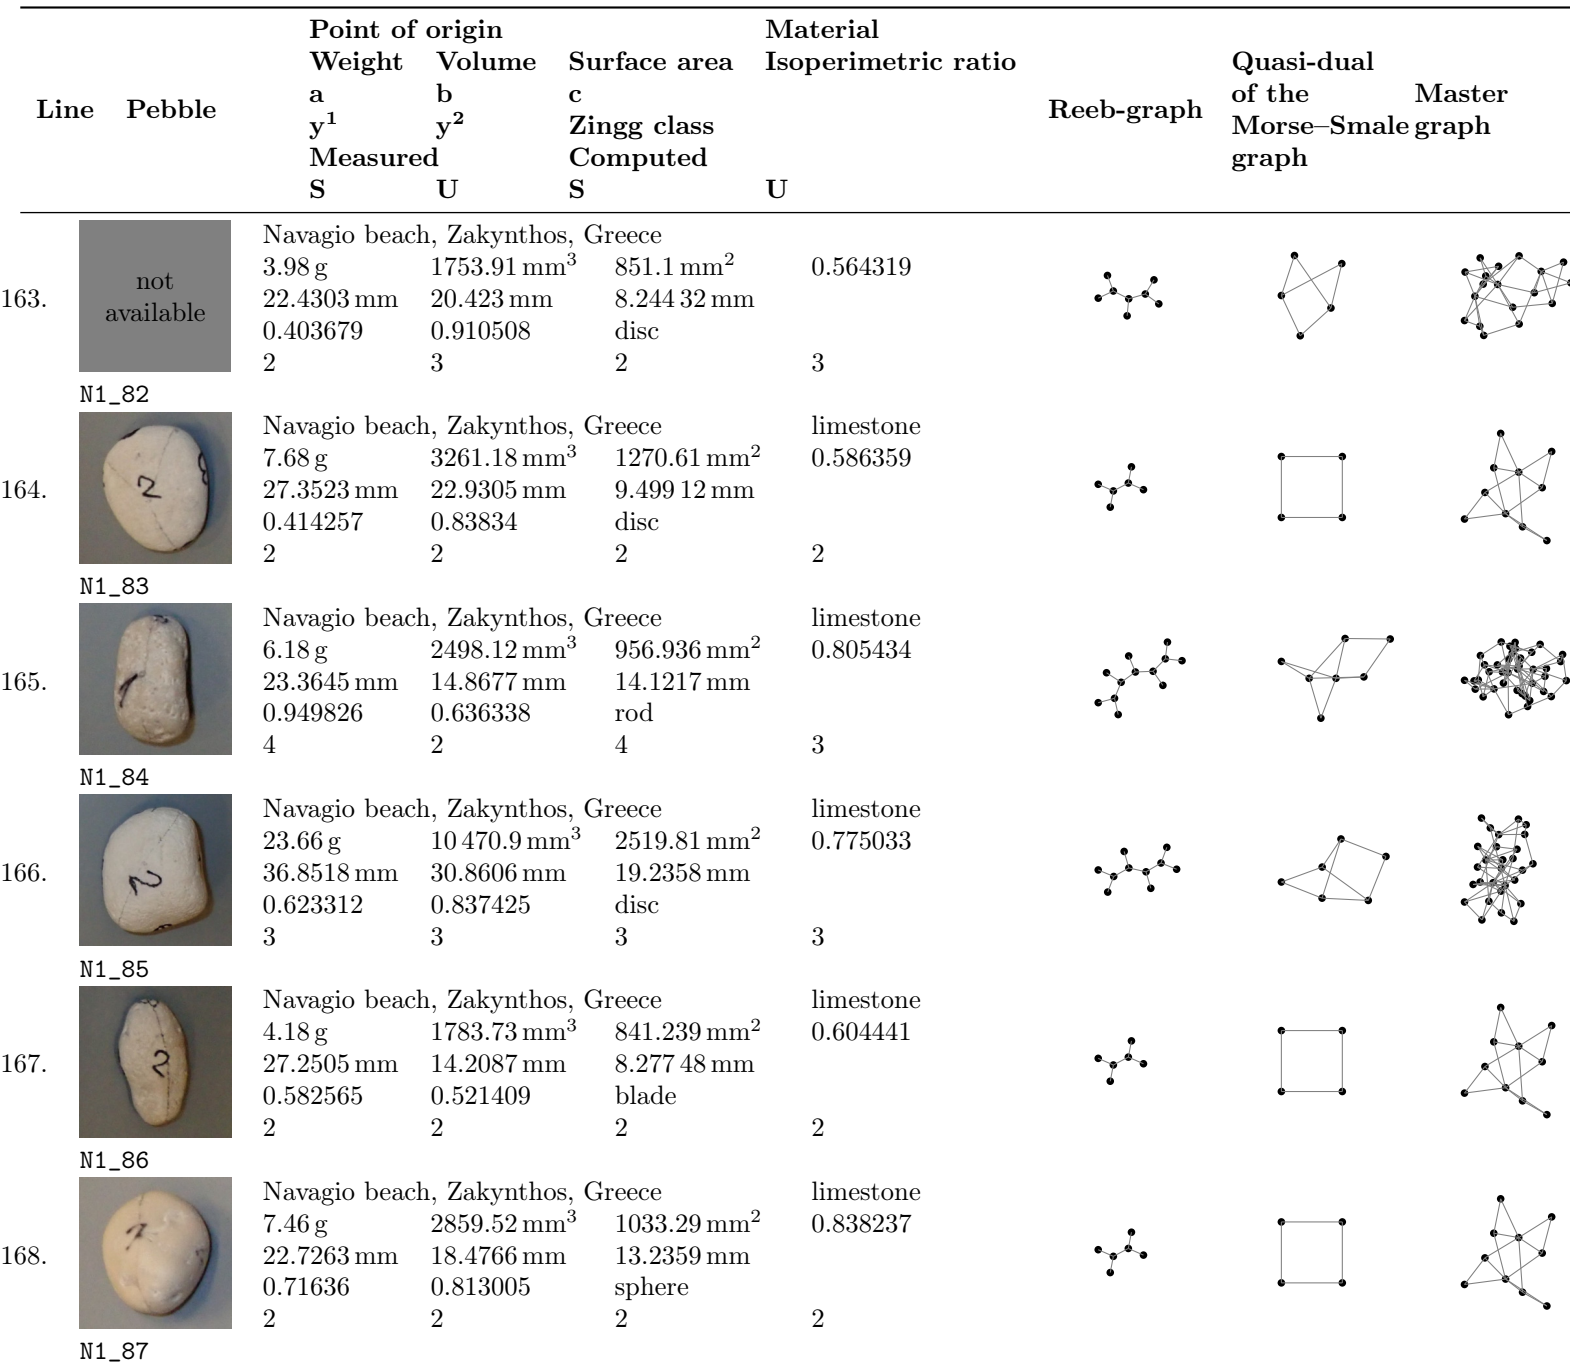   |
|      |                                                                                     | 6.18 g                           | 2498.12 mm <sup>3</sup>  | 956.936 mm <sup>2</sup>      |                       |                                                                                       |                                                                                       |                                                                                       |
|      |                                                                                     | 23.3645 mm                       | 14.8677 mm               | 14.1217 mm                   |                       |                                                                                       |                                                                                       |                                                                                       |
|      |                                                                                     | 0.949826                         | 0.636338                 | rod                          |                       |                                                                                       |                                                                                       |                                                                                       |
|      |                                                                                     | 4                                | 2                        | 4                            |                       |                                                                                       |                                                                                       |                                                                                       |
|      | N1_84                                                                               |                                  |                          |                              | 3                     |                                                                                       |                                                                                       |                                                                                       |
| 166. | 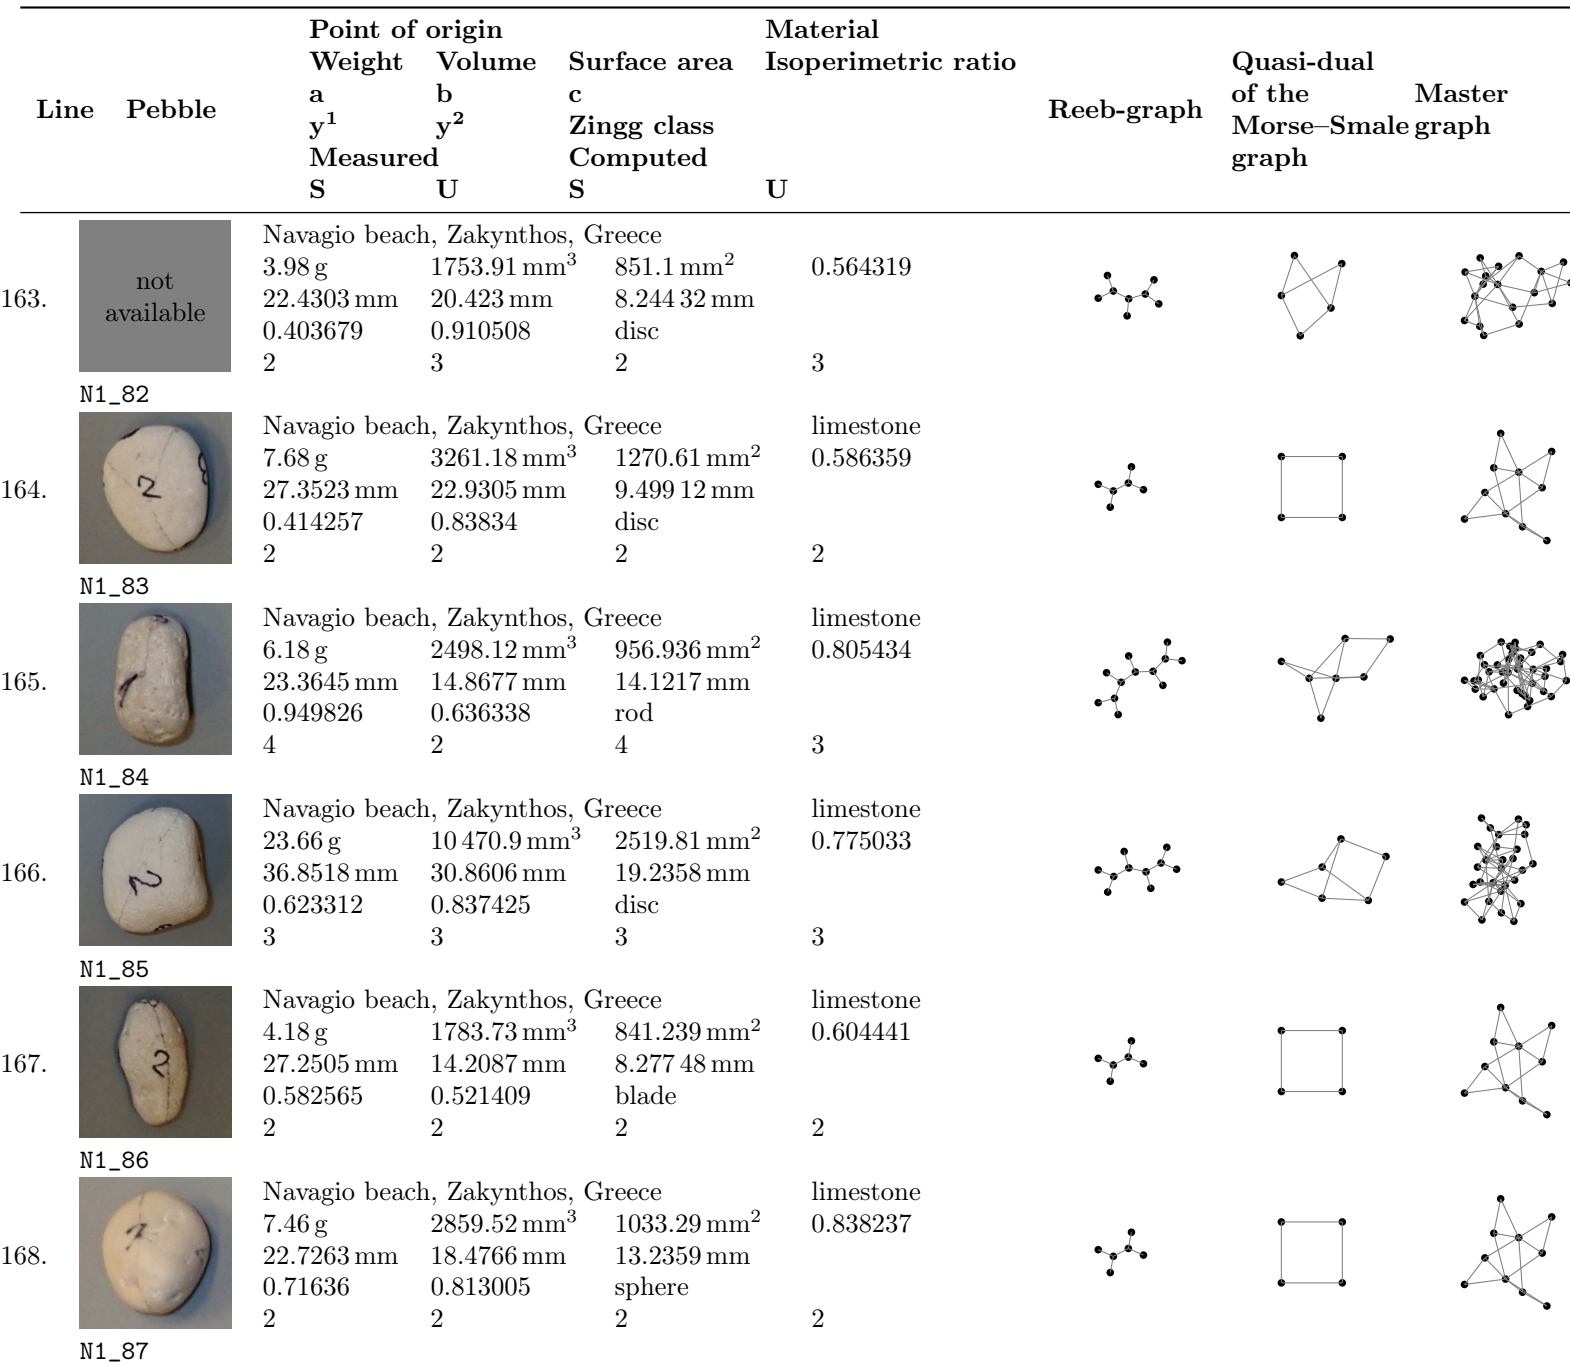  | Navagio beach, Zakynthos, Greece |                          |                              | limestone<br>0.775033 | 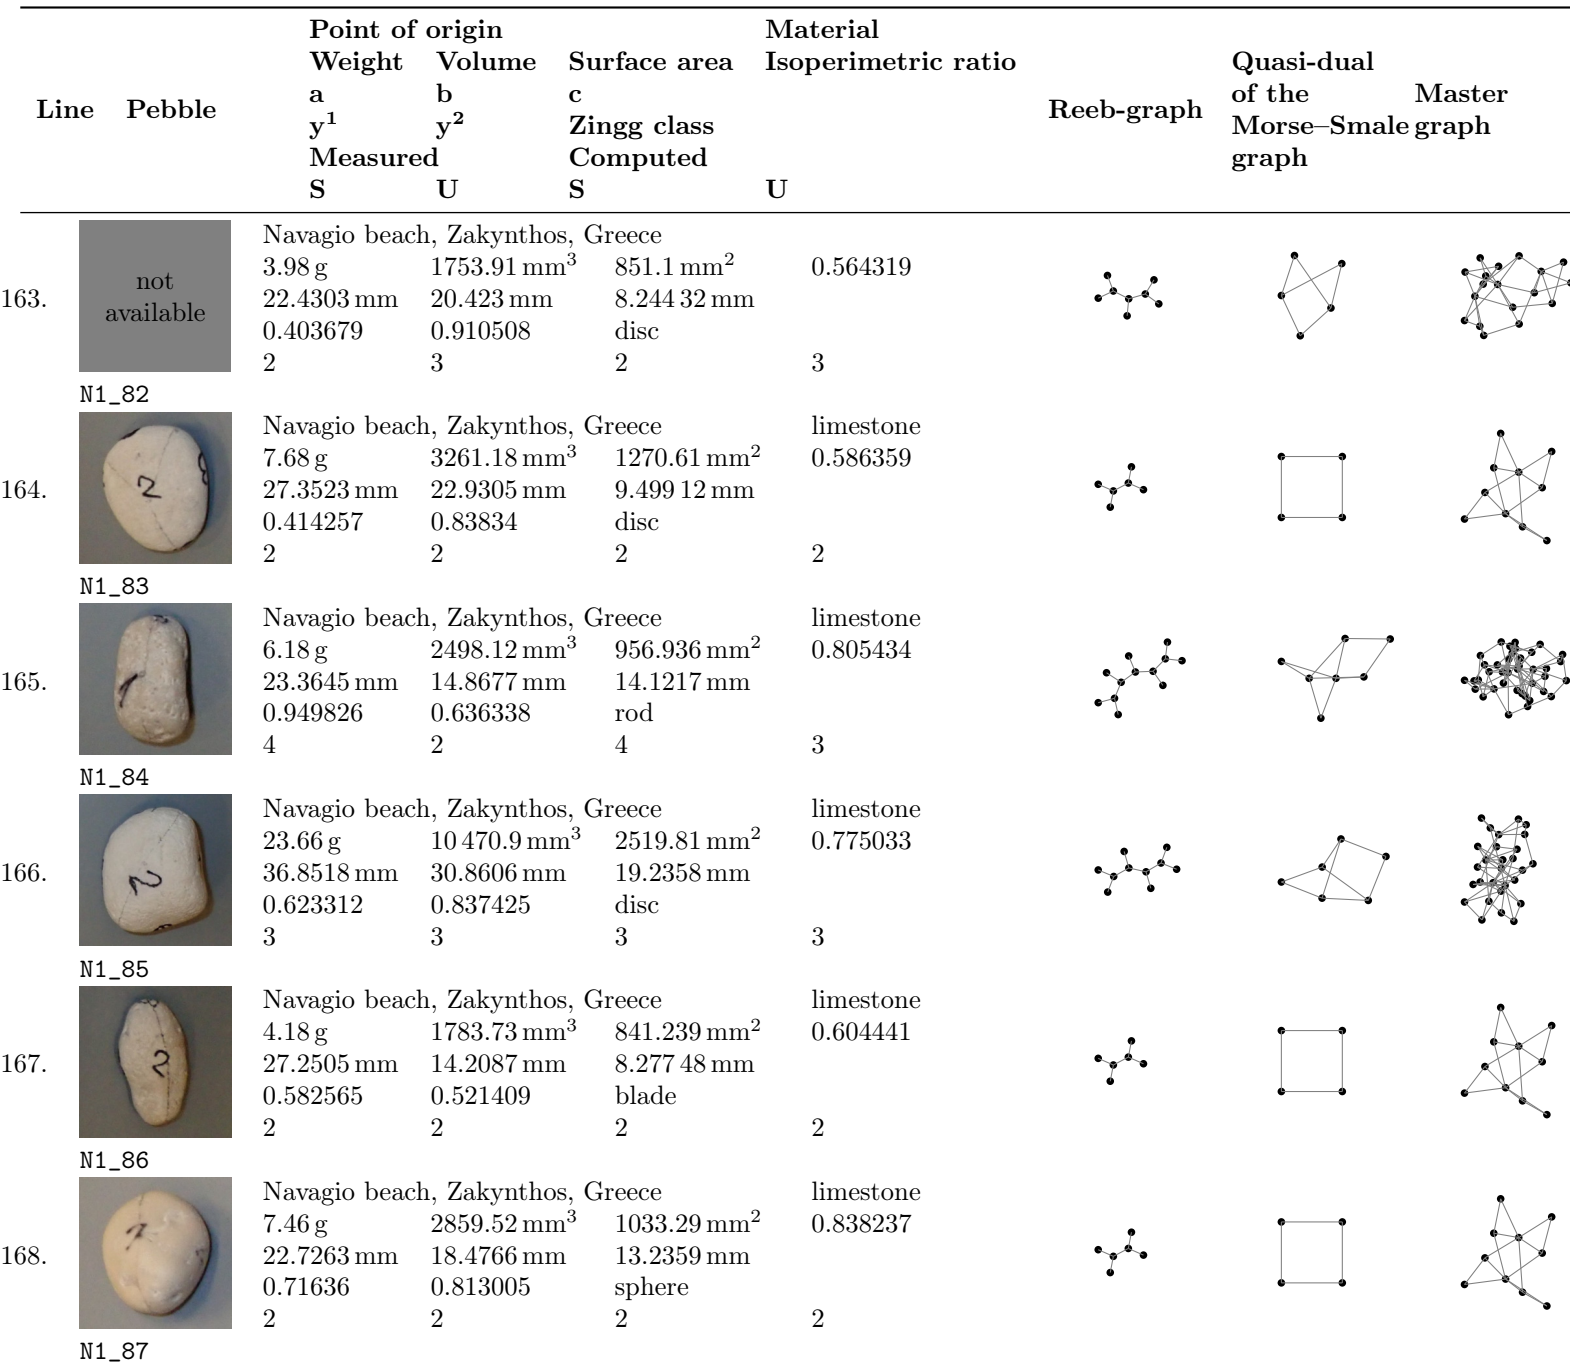  | 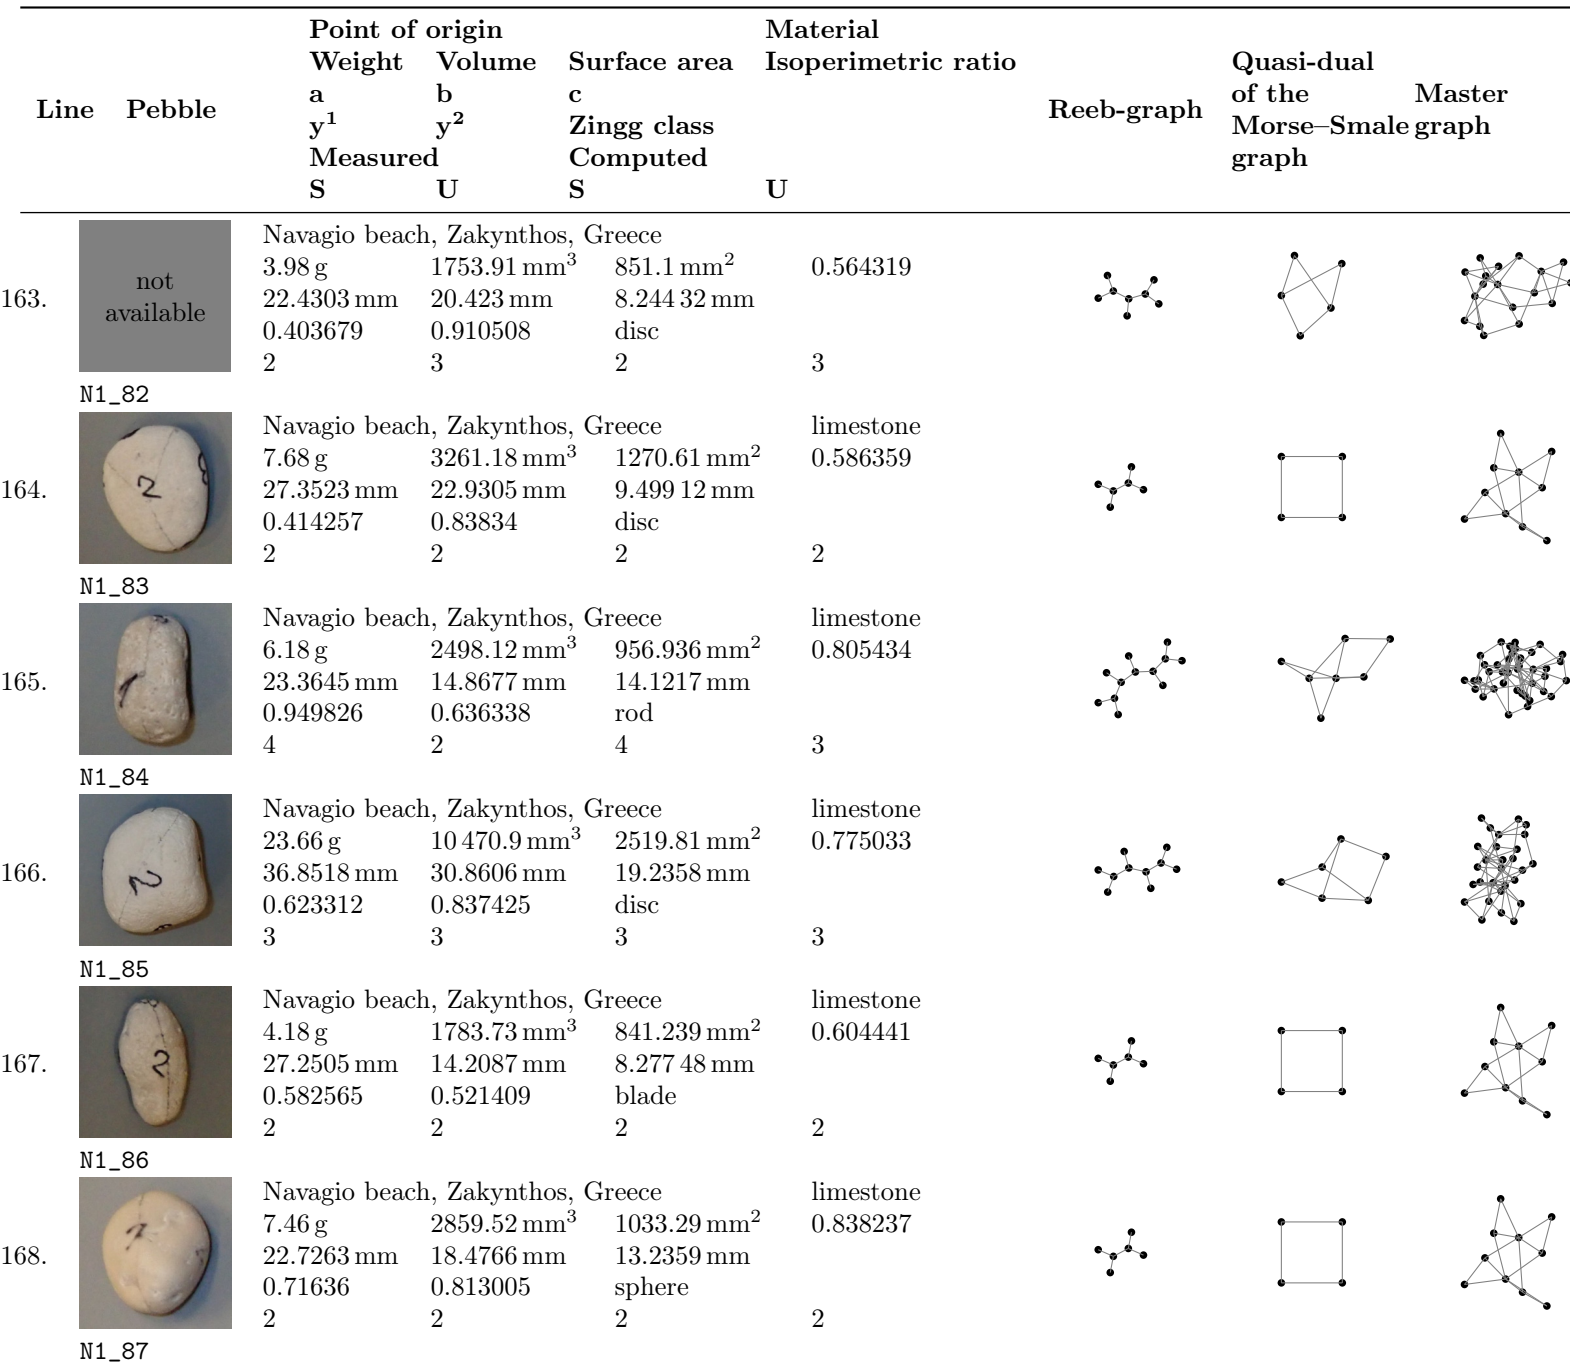  | 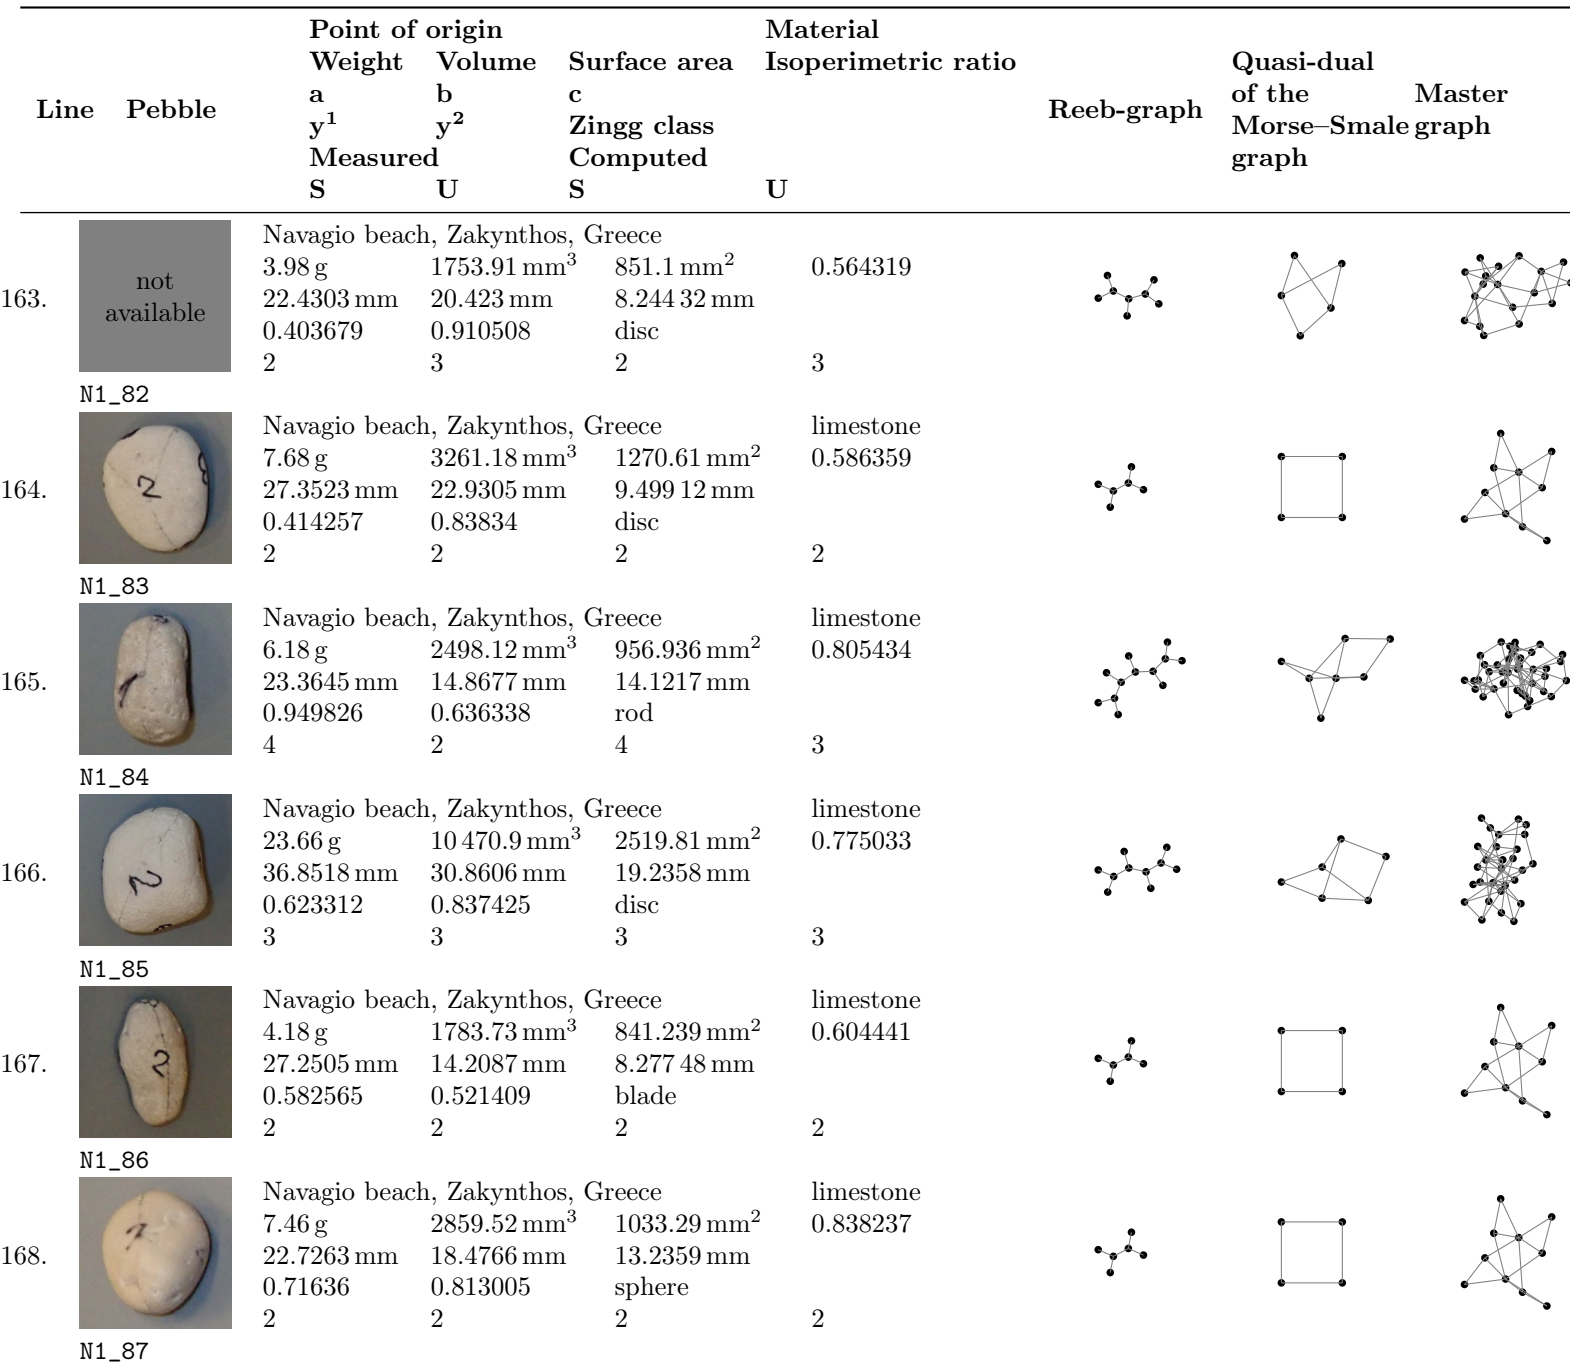  |
|      |                                                                                     | 23.66 g                          | 10 470.9 mm <sup>3</sup> | 2519.81 mm <sup>2</sup>      |                       |                                                                                       |                                                                                       |                                                                                       |
|      |                                                                                     | 36.8518 mm                       | 30.8606 mm               | 19.2358 mm                   |                       |                                                                                       |                                                                                       |                                                                                       |
|      |                                                                                     | 0.623312                         | 0.837425                 | disc                         |                       |                                                                                       |                                                                                       |                                                                                       |
|      |                                                                                     | 3                                | 3                        | 3                            |                       |                                                                                       |                                                                                       |                                                                                       |
|      | N1_85                                                                               |                                  |                          |                              | 3                     |                                                                                       |                                                                                       |                                                                                       |
| 167. | 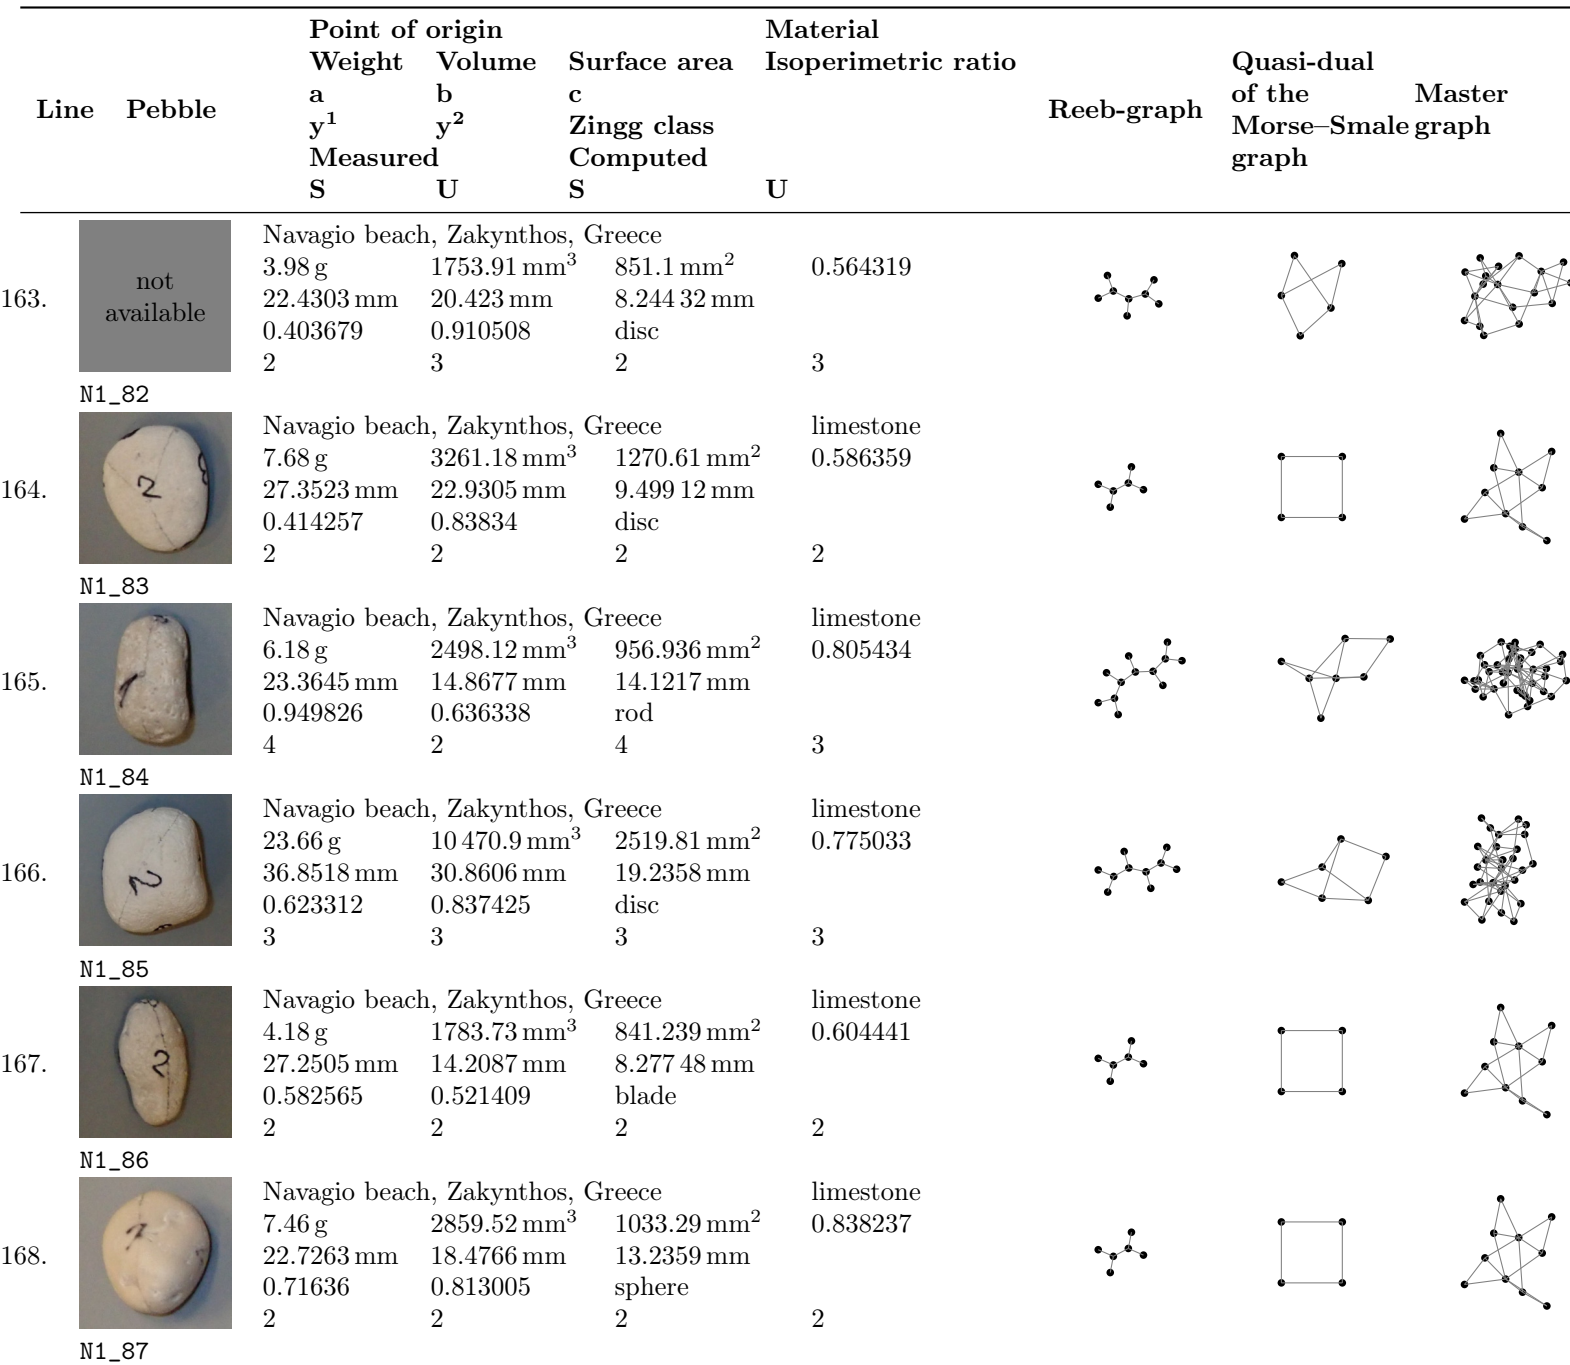 | Navagio beach, Zakynthos, Greece |                          |                              | limestone<br>0.604441 | 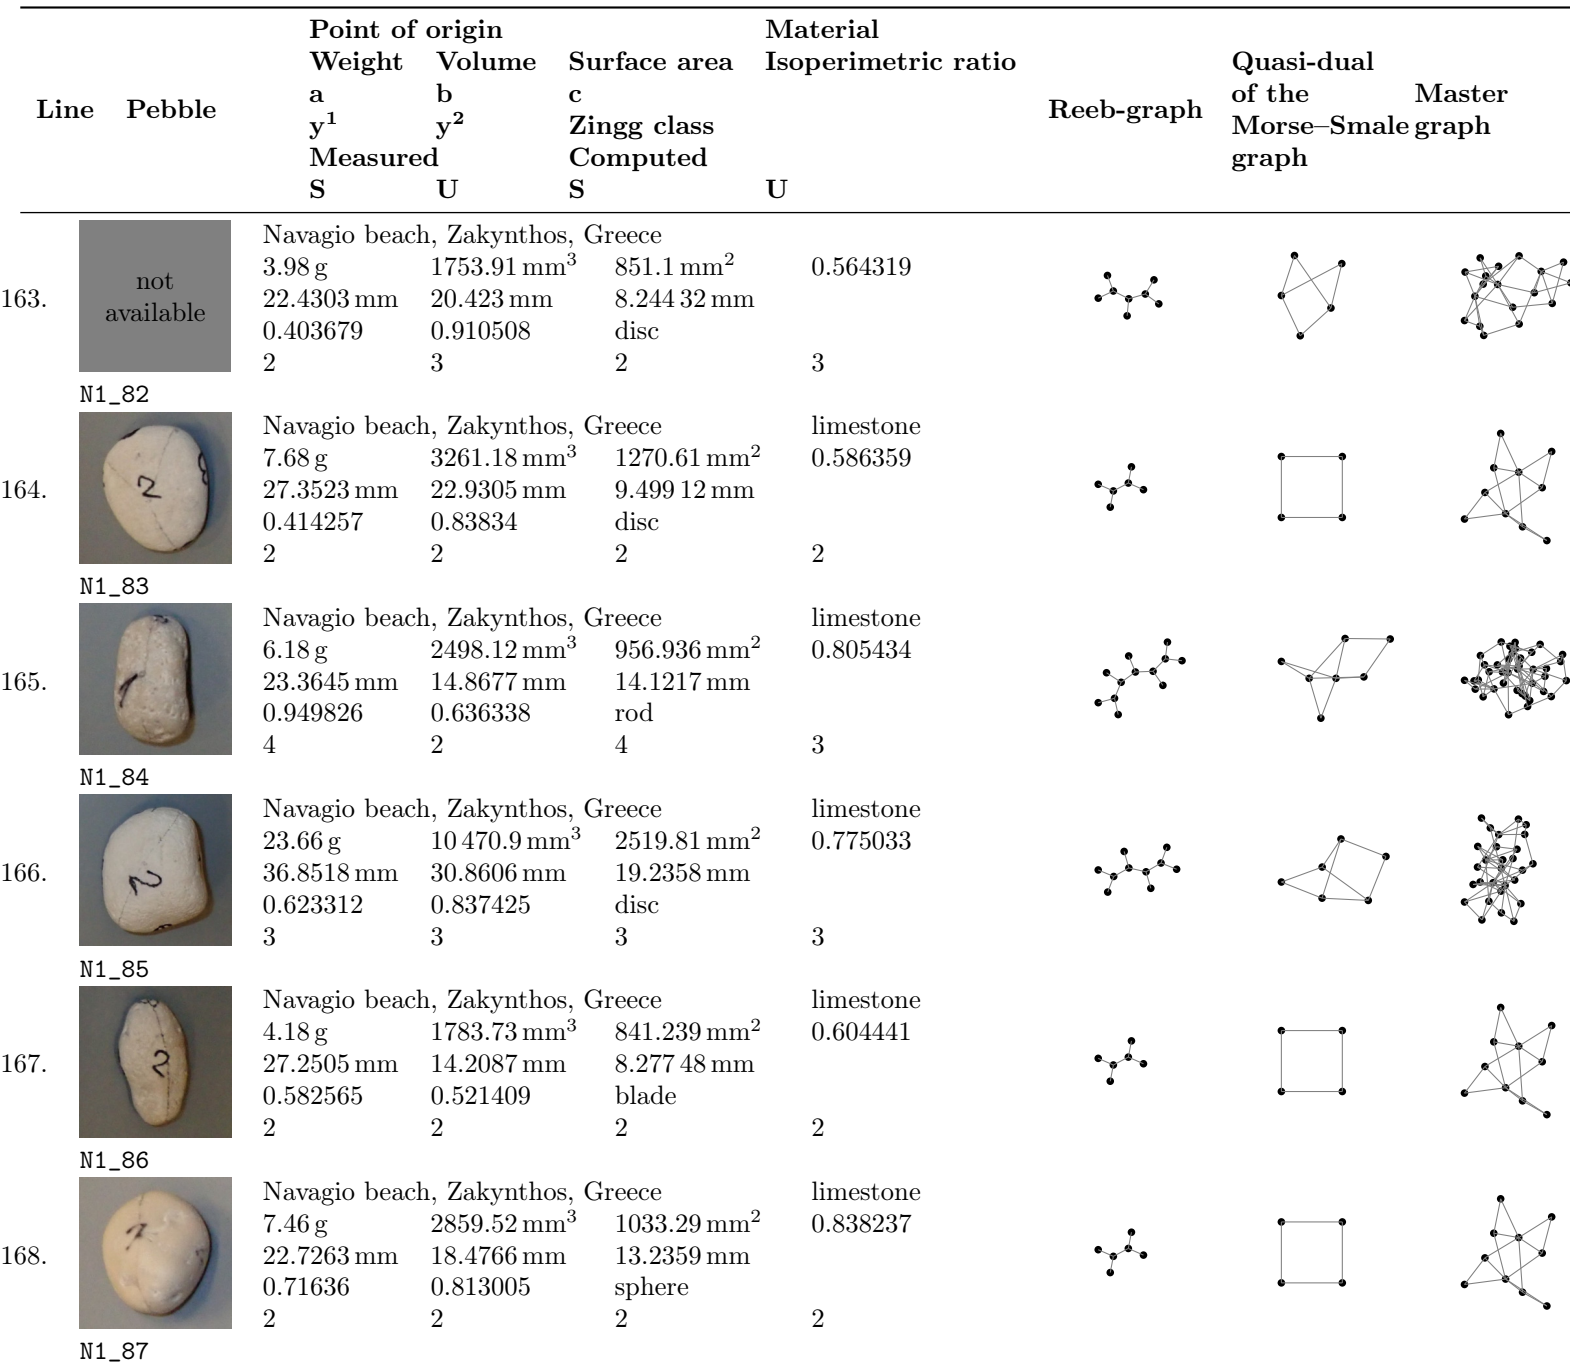 | 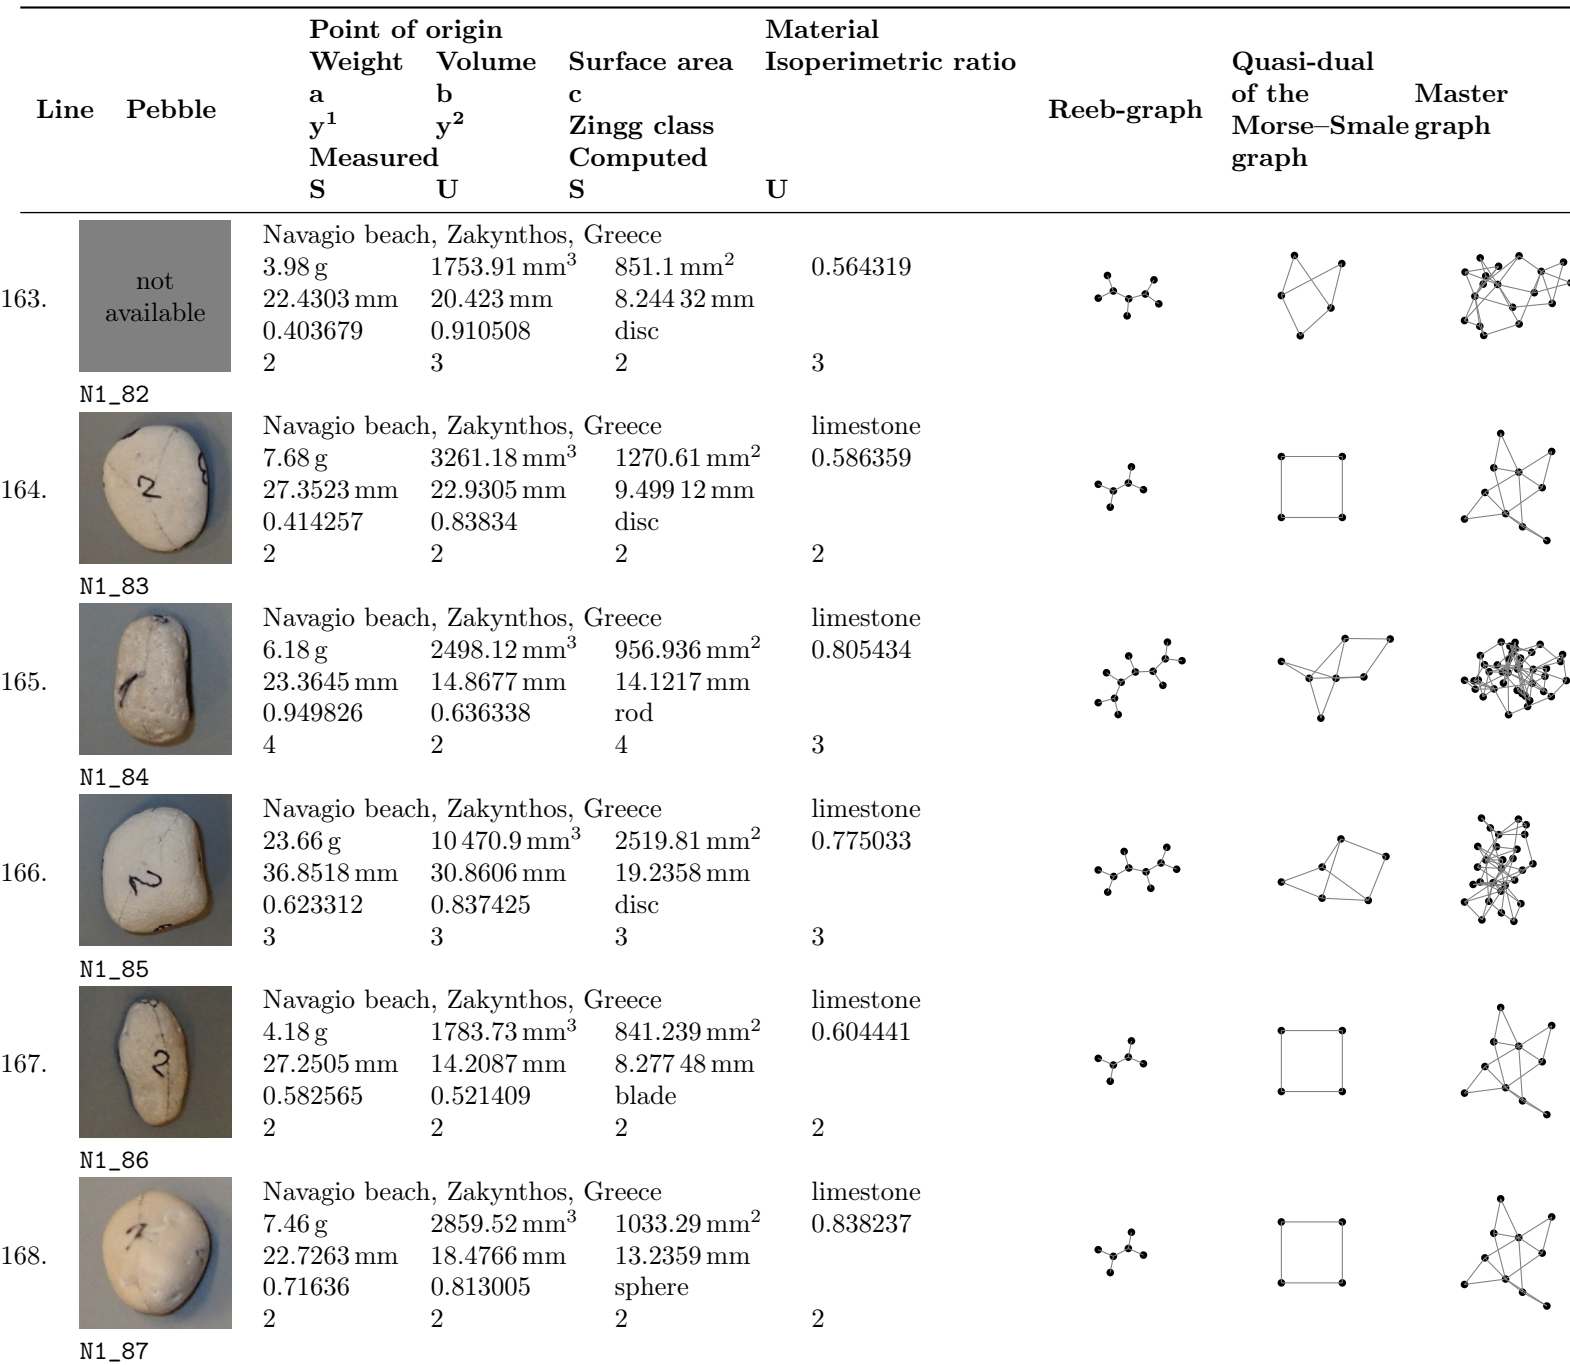 | 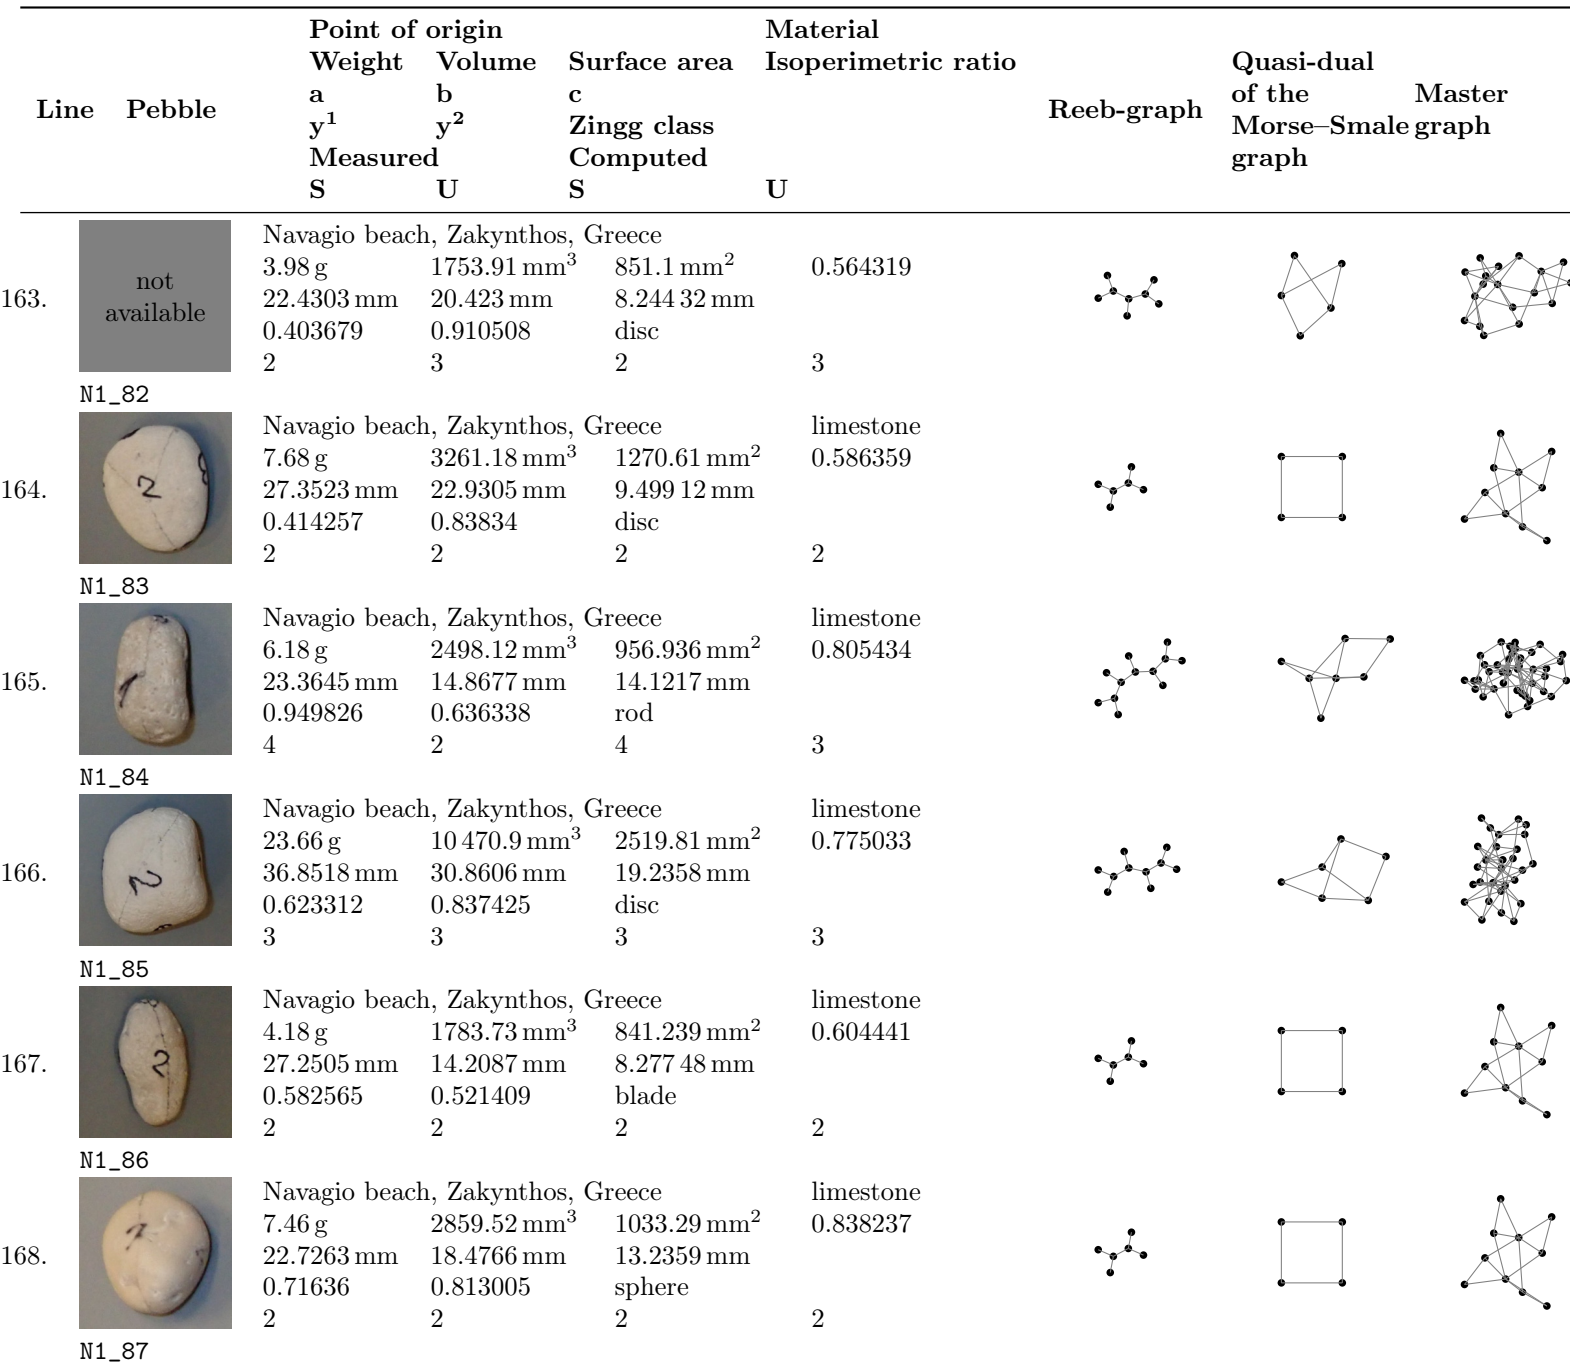 |
|      |                                                                                     | 4.18 g                           | 1783.73 mm <sup>3</sup>  | 841.239 mm <sup>2</sup>      |                       |                                                                                       |                                                                                       |                                                                                       |
|      |                                                                                     | 27.2505 mm                       | 14.2087 mm               | 8.277 48 mm                  |                       |                                                                                       |                                                                                       |                                                                                       |
|      |                                                                                     | 0.582565                         | 0.521409                 | blade                        |                       |                                                                                       |                                                                                       |                                                                                       |
|      |                                                                                     | 2                                | 2                        | 2                            |                       |                                                                                       |                                                                                       |                                                                                       |
|      | N1_86                                                                               |                                  |                          |                              | 2                     |                                                                                       |                                                                                       |                                                                                       |
| 168. | 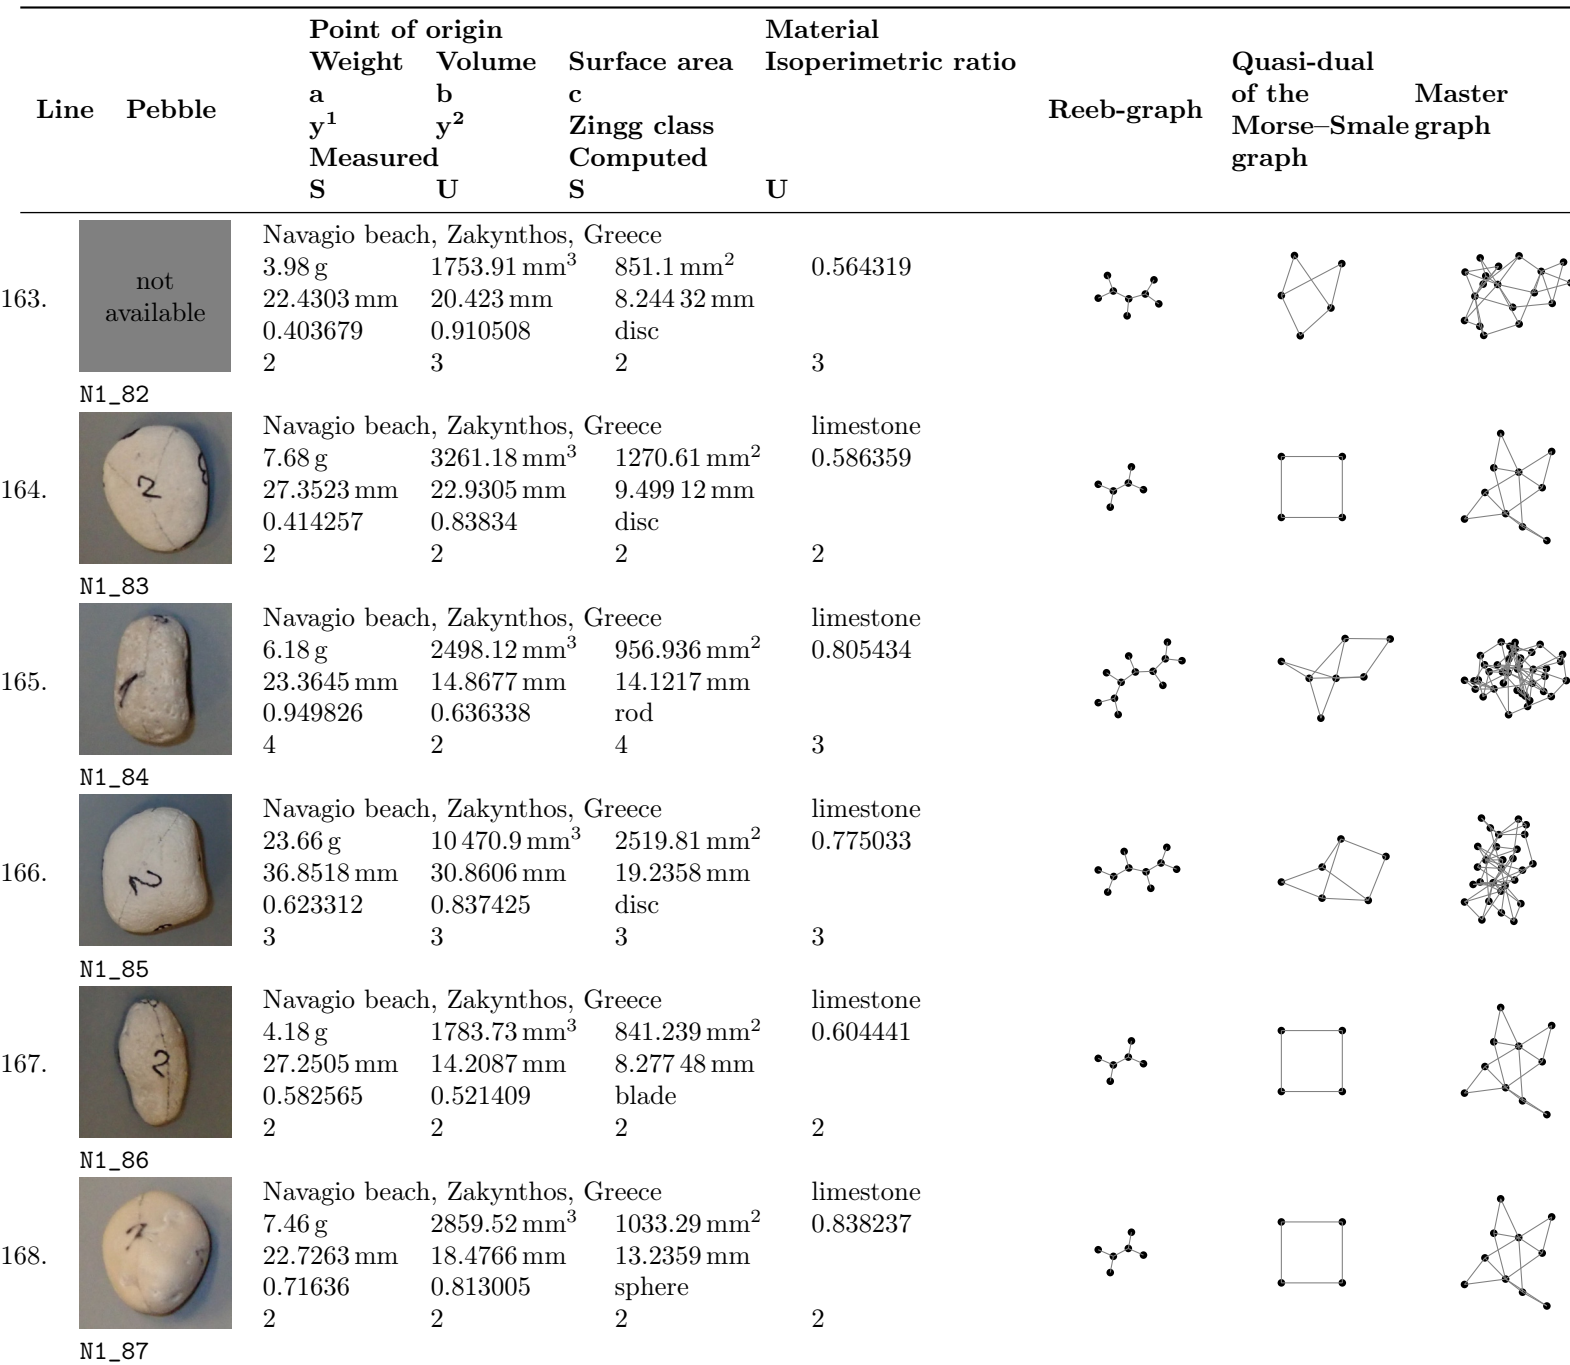 | Navagio beach, Zakynthos, Greece |                          |                              | limestone<br>0.838237 | 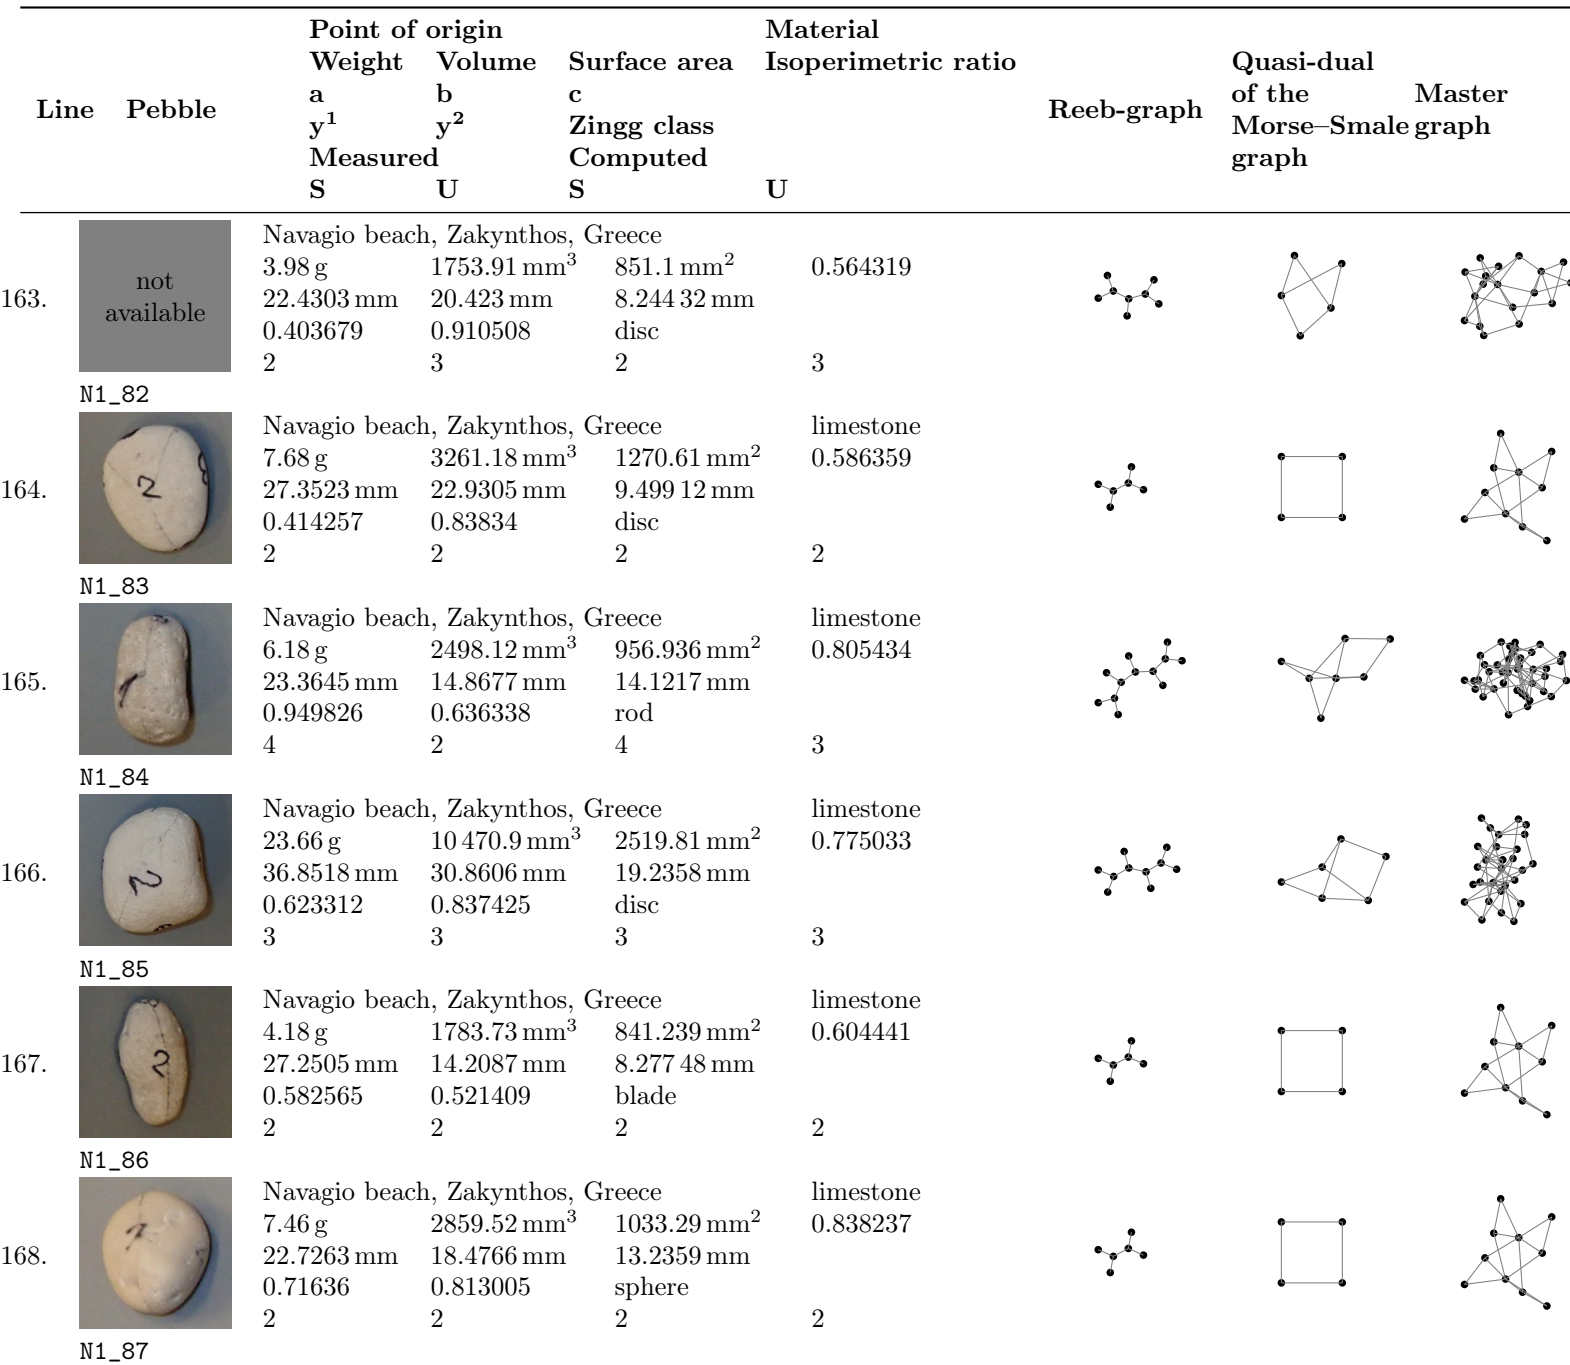 | 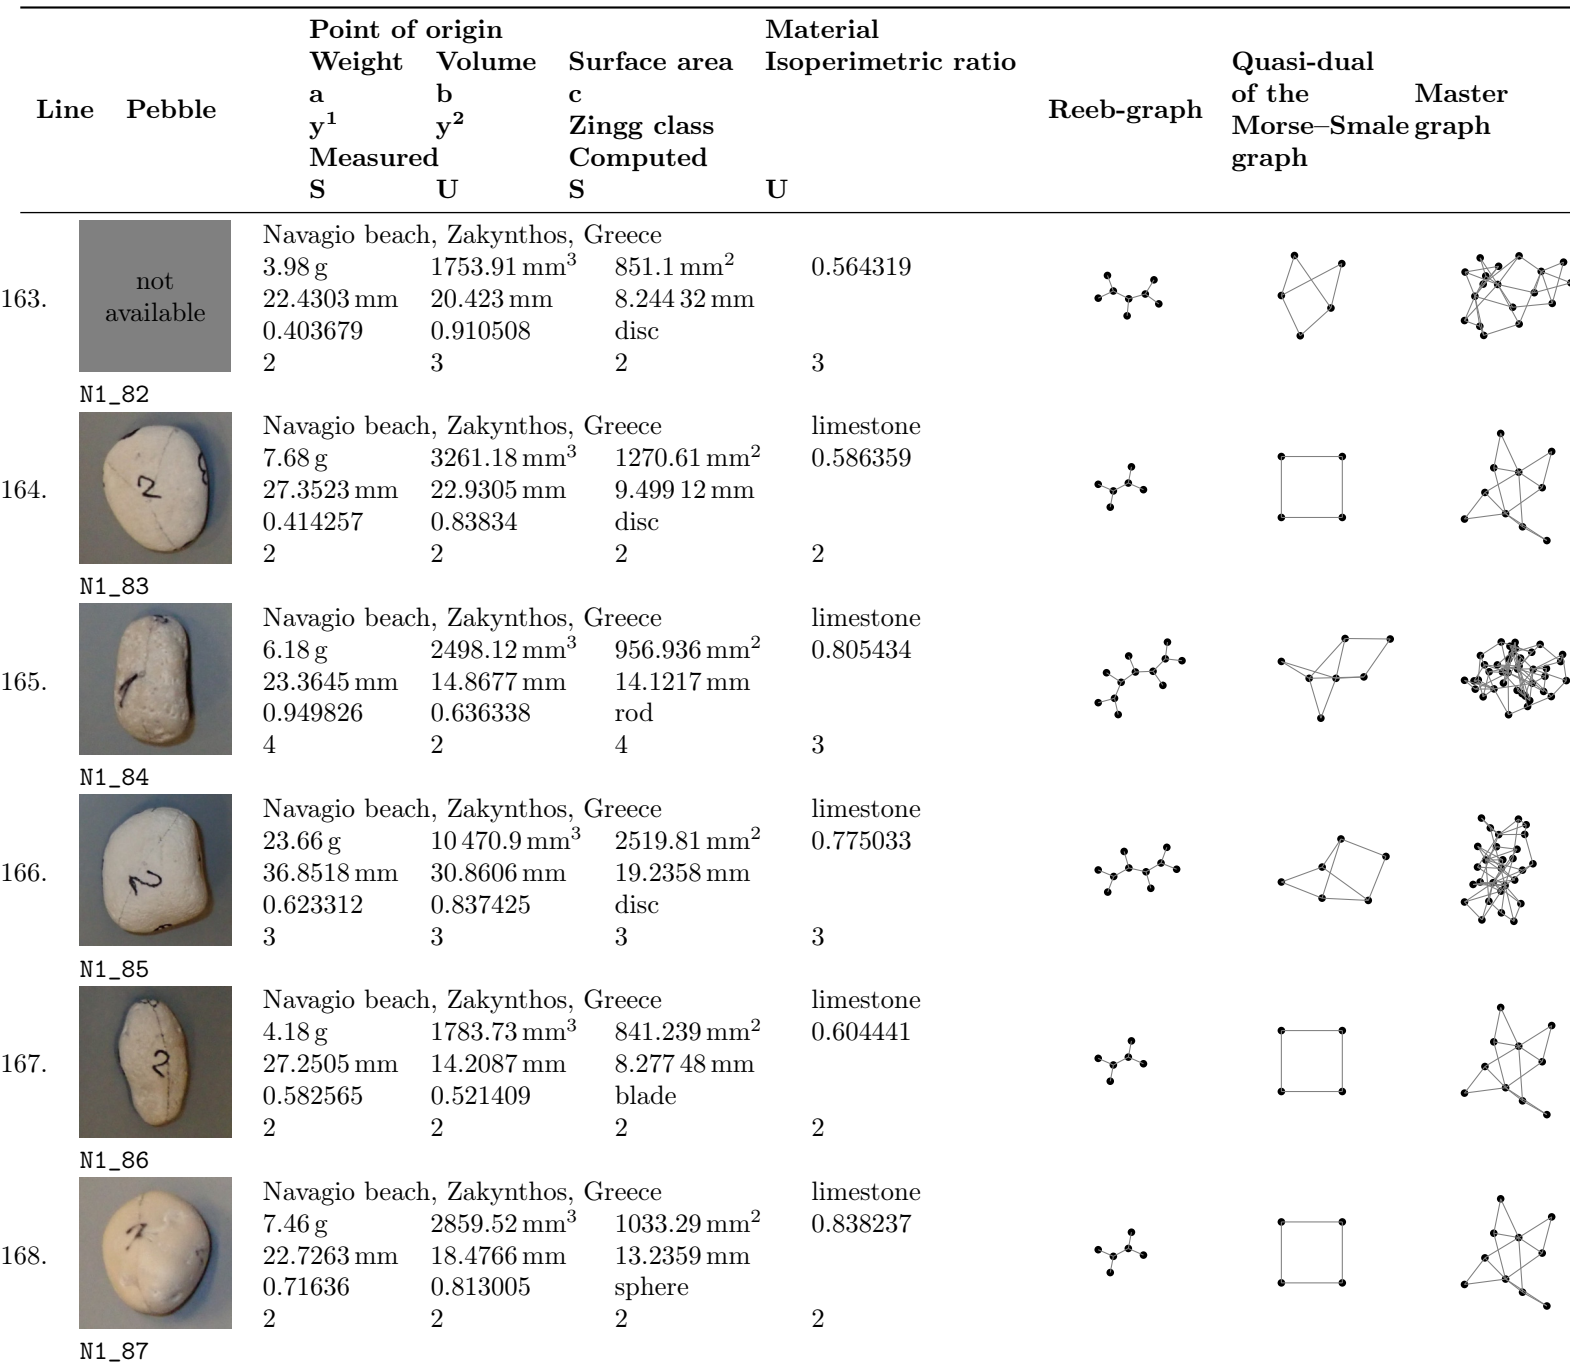 | 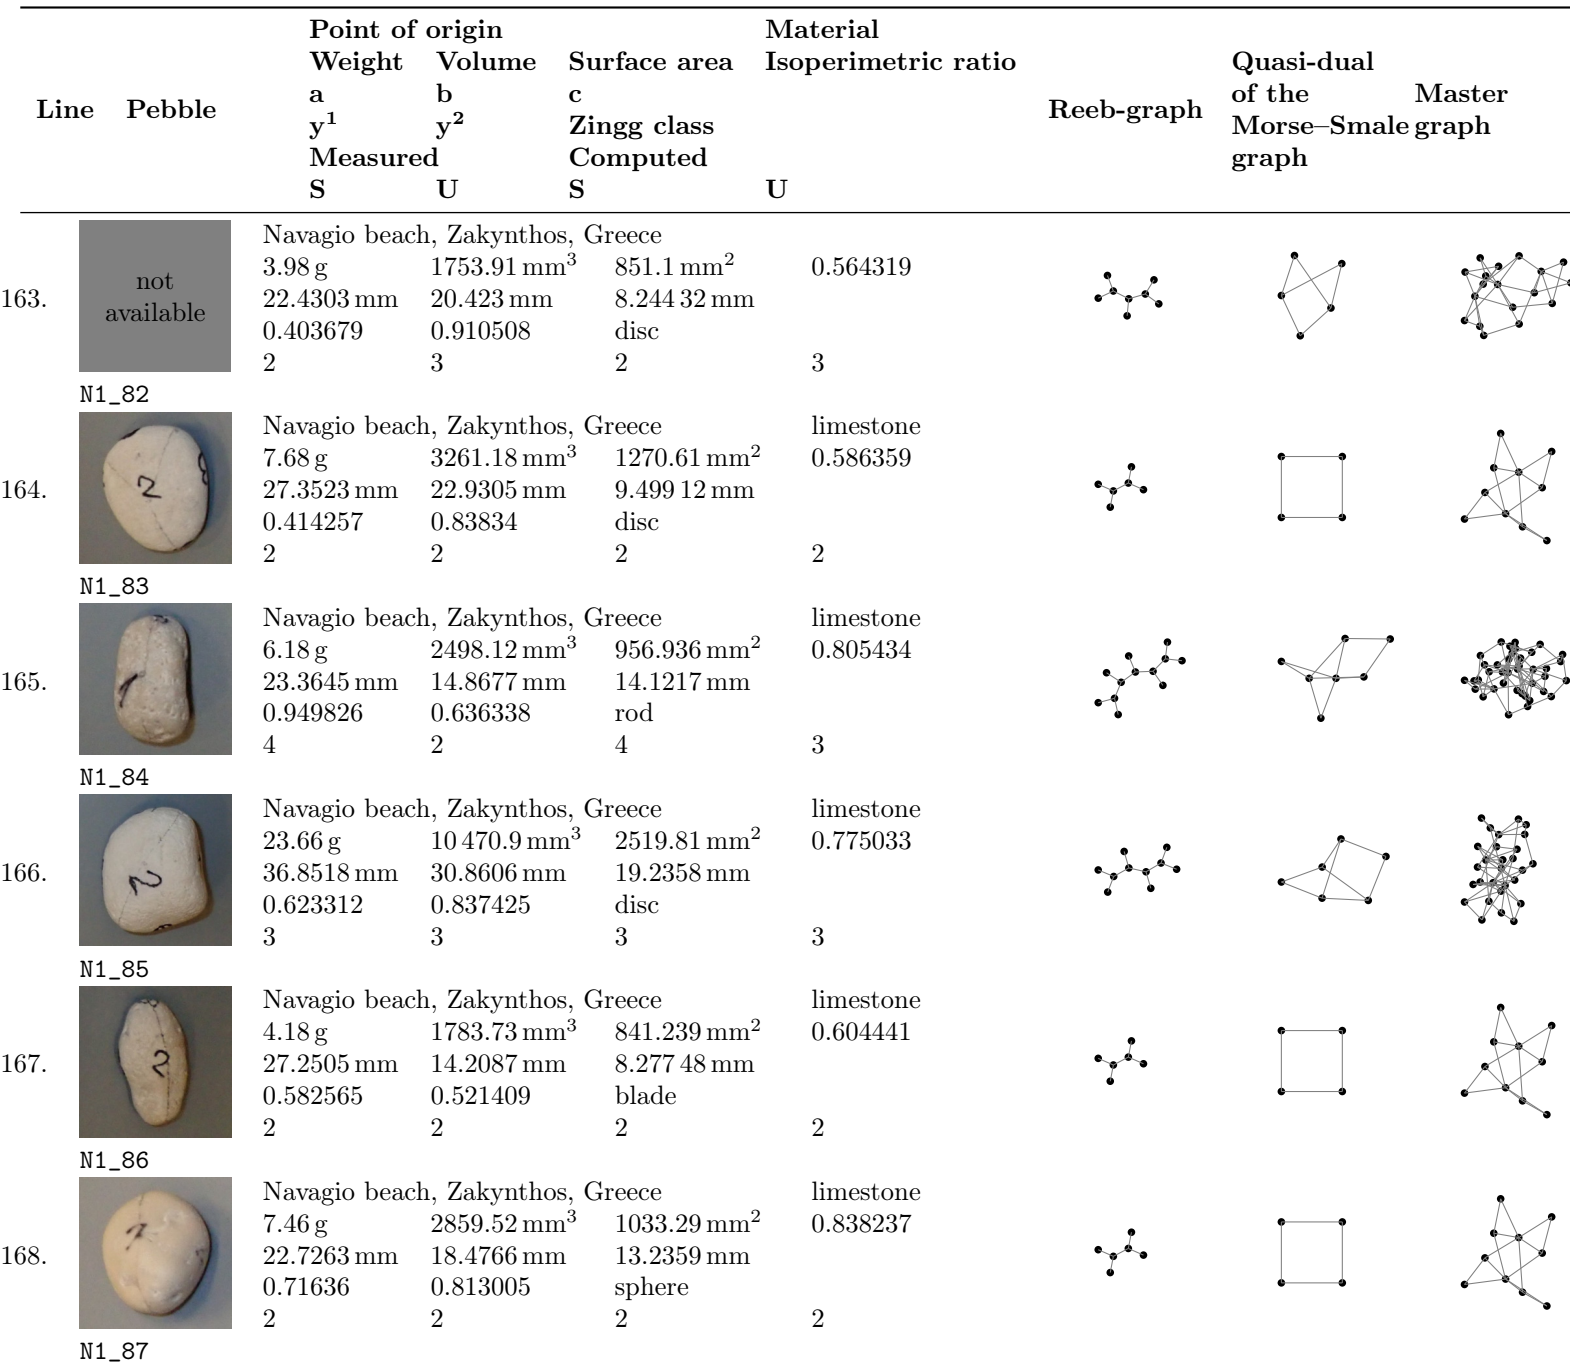 |
|      |                                                                                     | 7.46 g                           | 2859.52 mm <sup>3</sup>  | 1033.29 mm <sup>2</sup>      |                       |                                                                                       |                                                                                       |                                                                                       |
|      |                                                                                     | 22.7263 mm                       | 18.4766 mm               | 13.2359 mm                   |                       |                                                                                       |                                                                                       |                                                                                       |
|      |                                                                                     | 0.71636                          | 0.813005                 | sphere                       |                       |                                                                                       |                                                                                       |                                                                                       |
|      |                                                                                     | 2                                | 2                        | 2                            |                       |                                                                                       |                                                                                       |                                                                                       |
|      | N1_87                                                                               |                                  |                          |                              | 2                     |                                                                                       |                                                                                       |                                                                                       |

| Line | Pebble                                                                              | Point of origin                  |                         |                              | Material  | Isoperimetric ratio | Reeb-graph                                                                            | Quasi-dual<br>of the<br>Morse–Smale<br>graph                                          | Master<br>graph                                                                       |
|------|-------------------------------------------------------------------------------------|----------------------------------|-------------------------|------------------------------|-----------|---------------------|---------------------------------------------------------------------------------------|---------------------------------------------------------------------------------------|---------------------------------------------------------------------------------------|
|      |                                                                                     | Weight                           | Volume                  | Surface area                 |           |                     |                                                                                       |                                                                                       |                                                                                       |
|      |                                                                                     | a                                | b                       | c                            |           |                     |                                                                                       |                                                                                       |                                                                                       |
|      |                                                                                     | y <sup>1</sup><br>Measured<br>S  | y <sup>2</sup><br>U     | Zingg class<br>Computed<br>S |           |                     |                                                                                       |                                                                                       |                                                                                       |
| 169. | 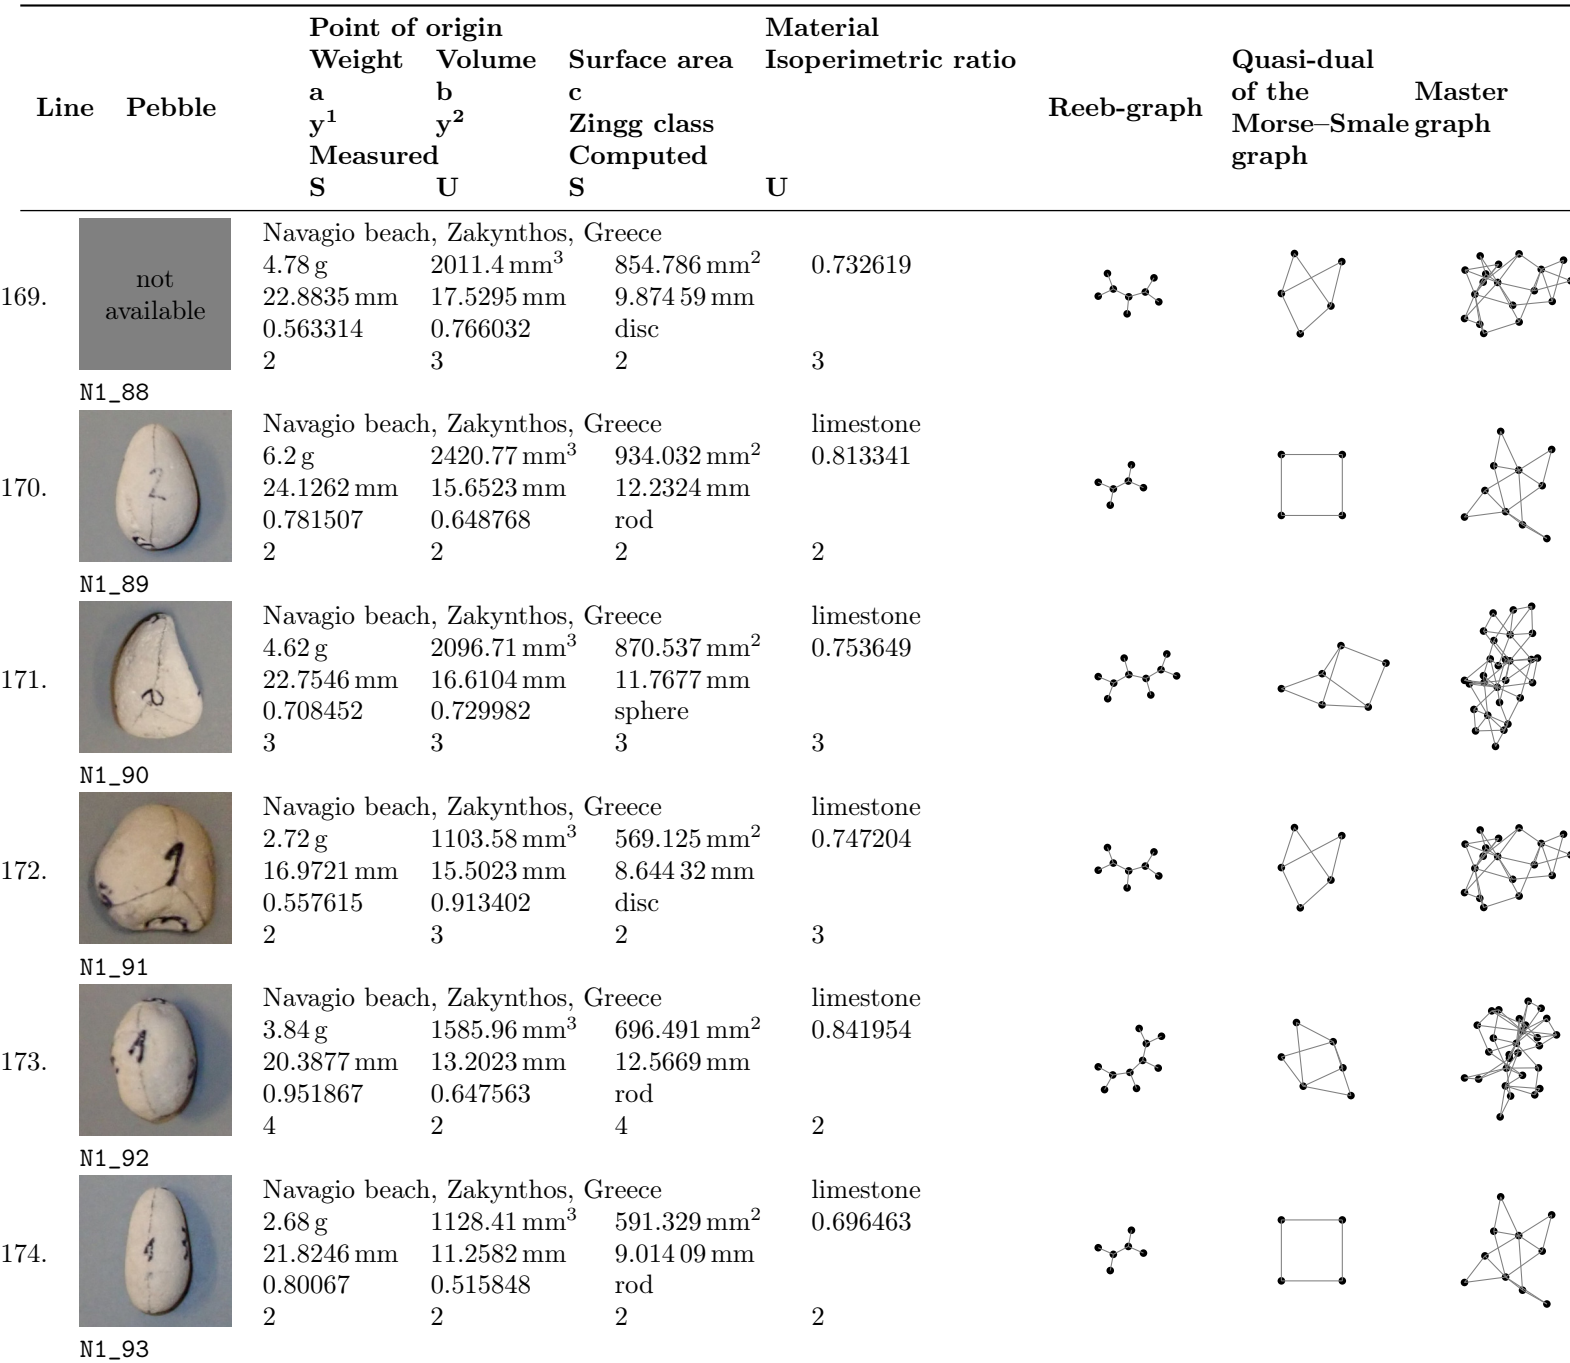   | Navagio beach, Zakynthos, Greece |                         |                              | limestone | 0.732619            | 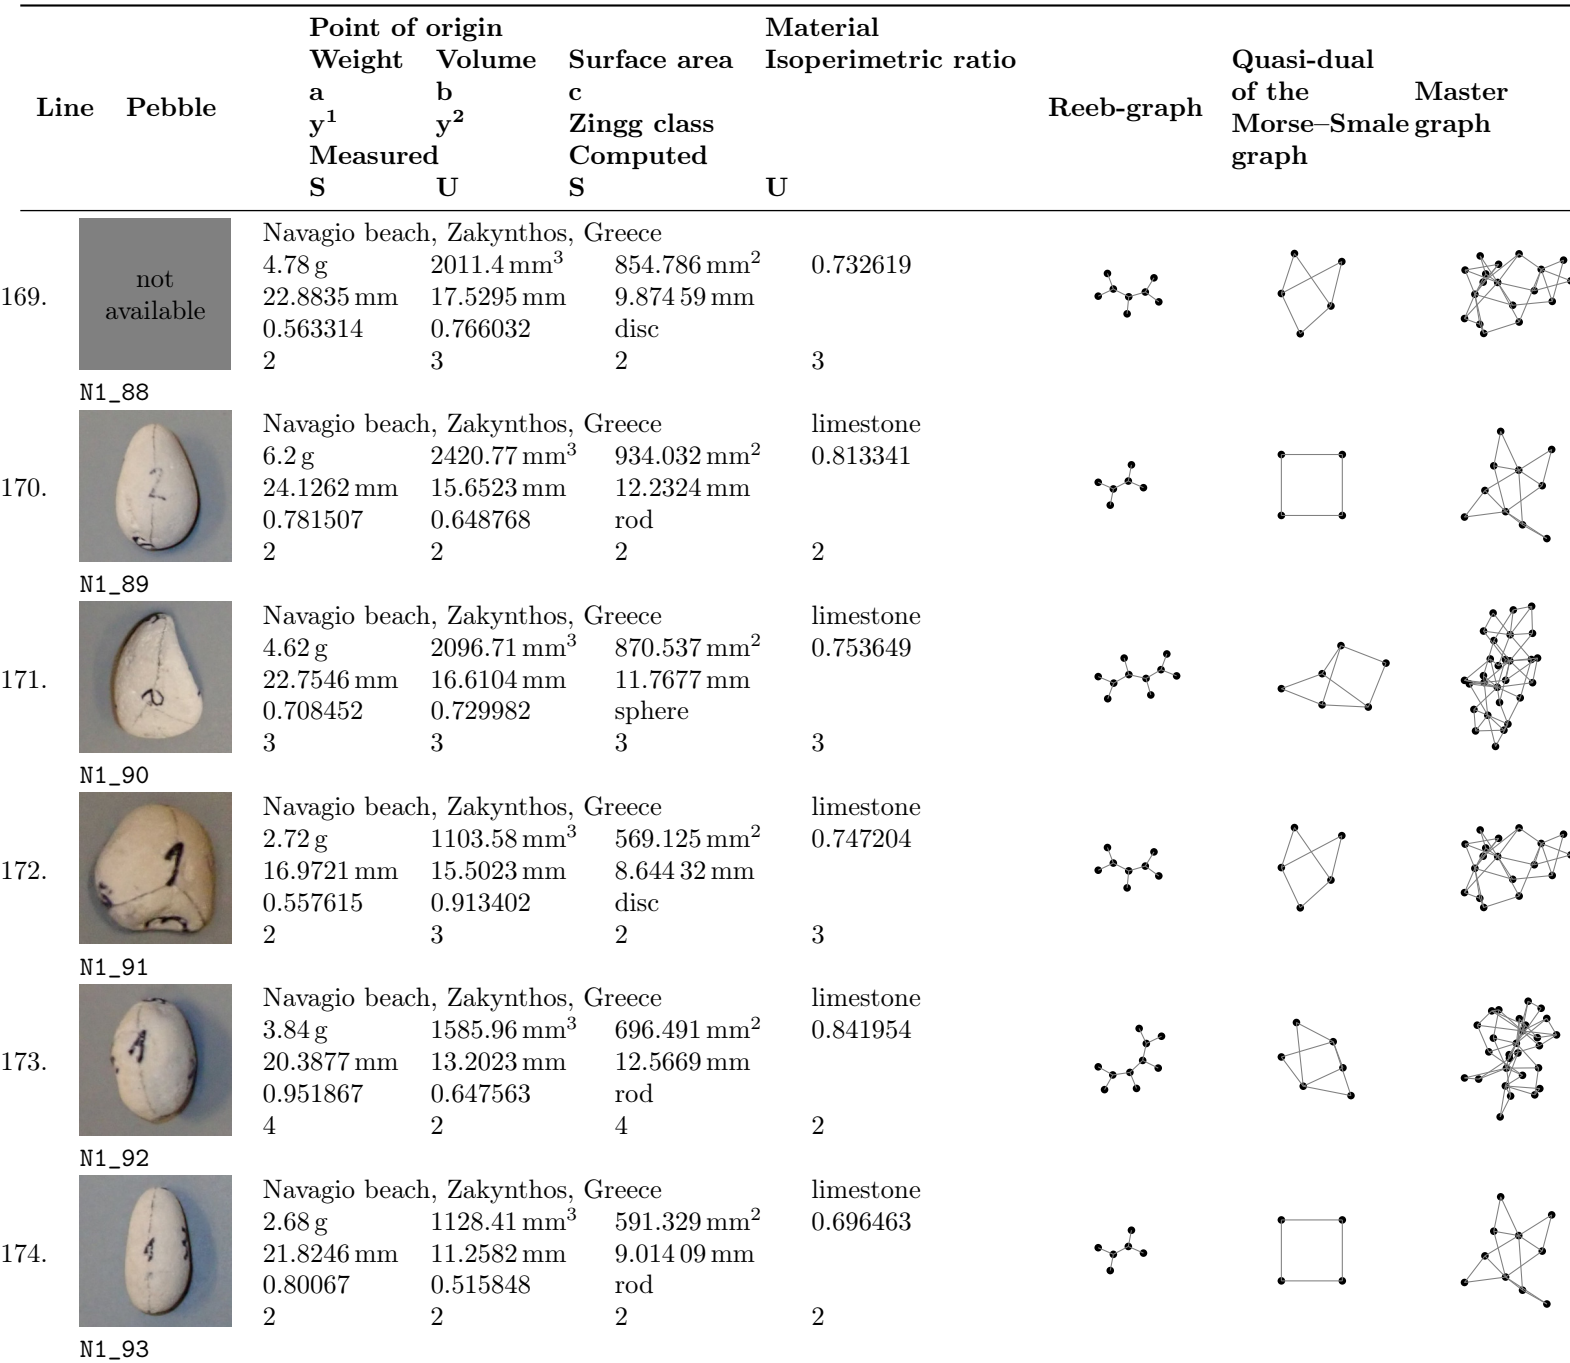   | 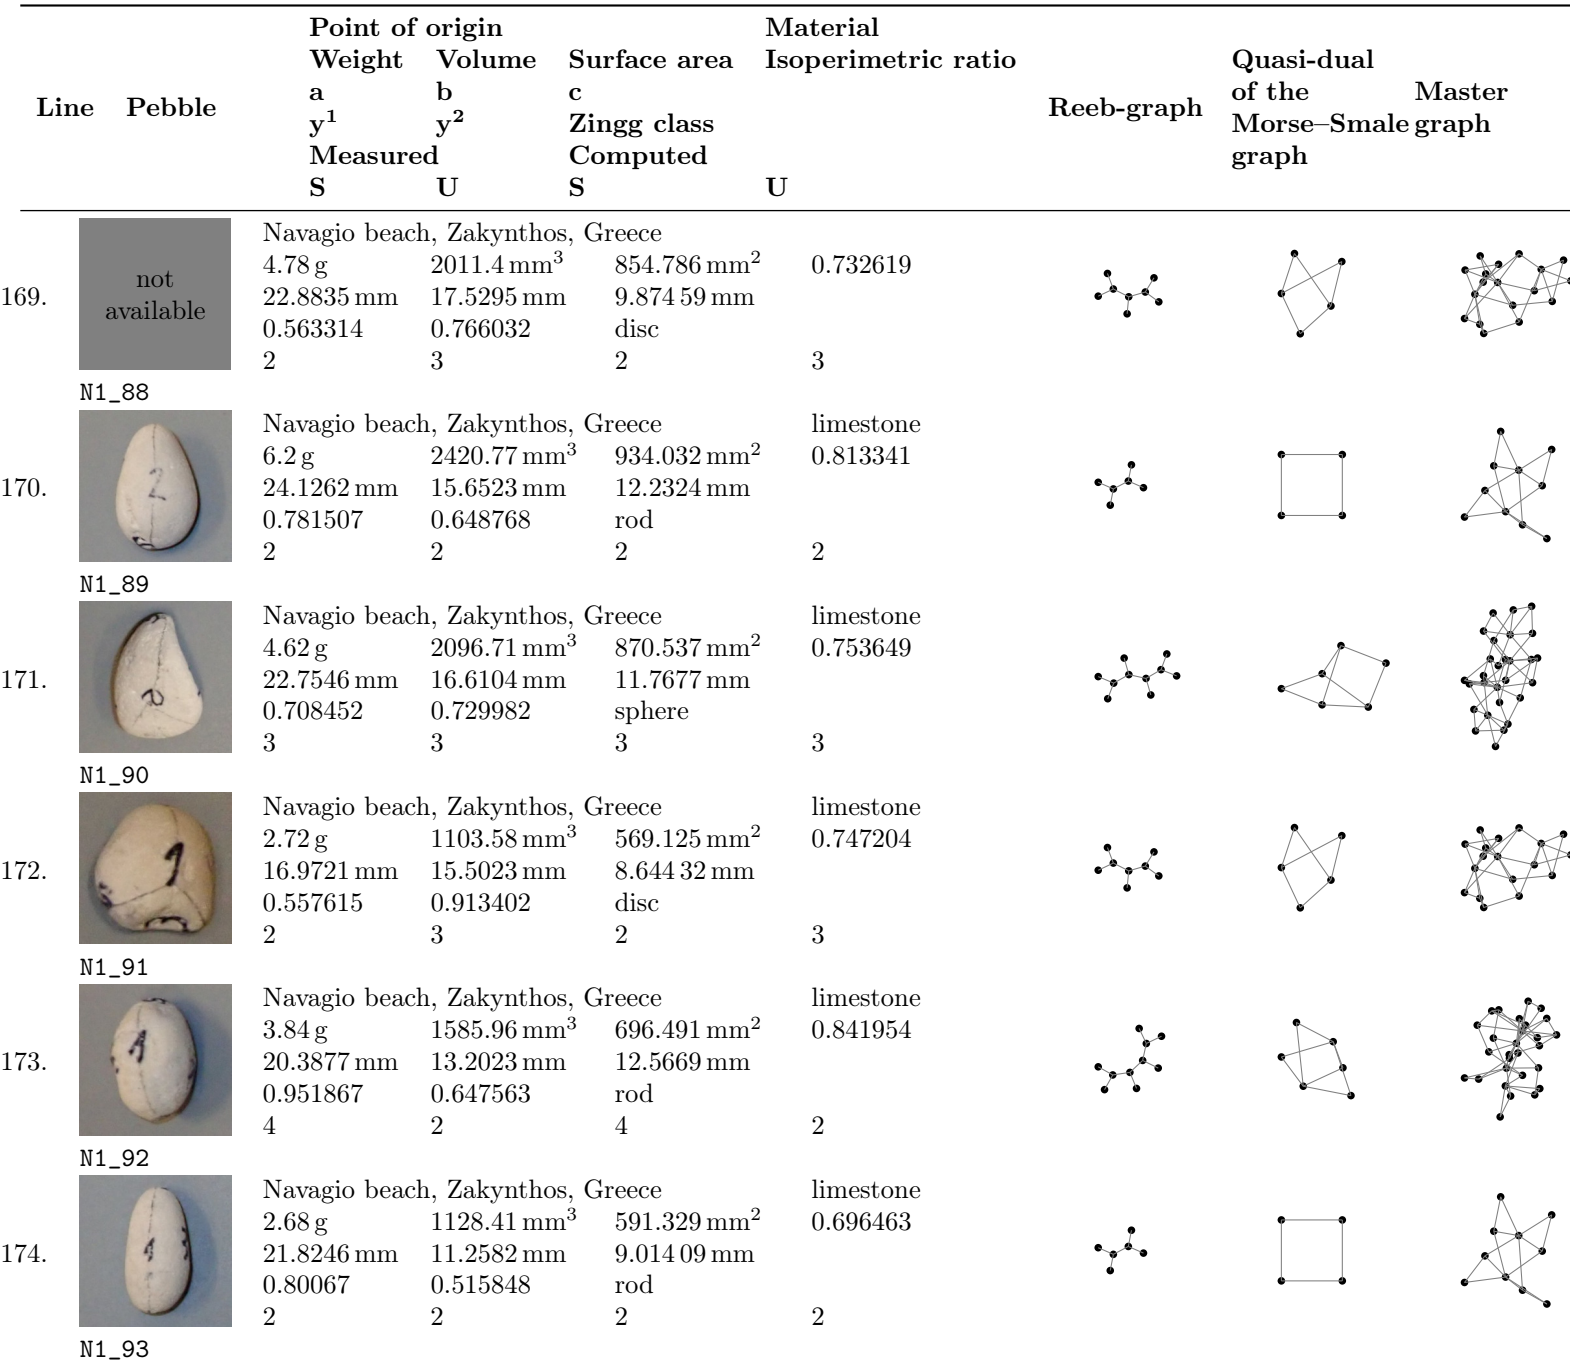   | 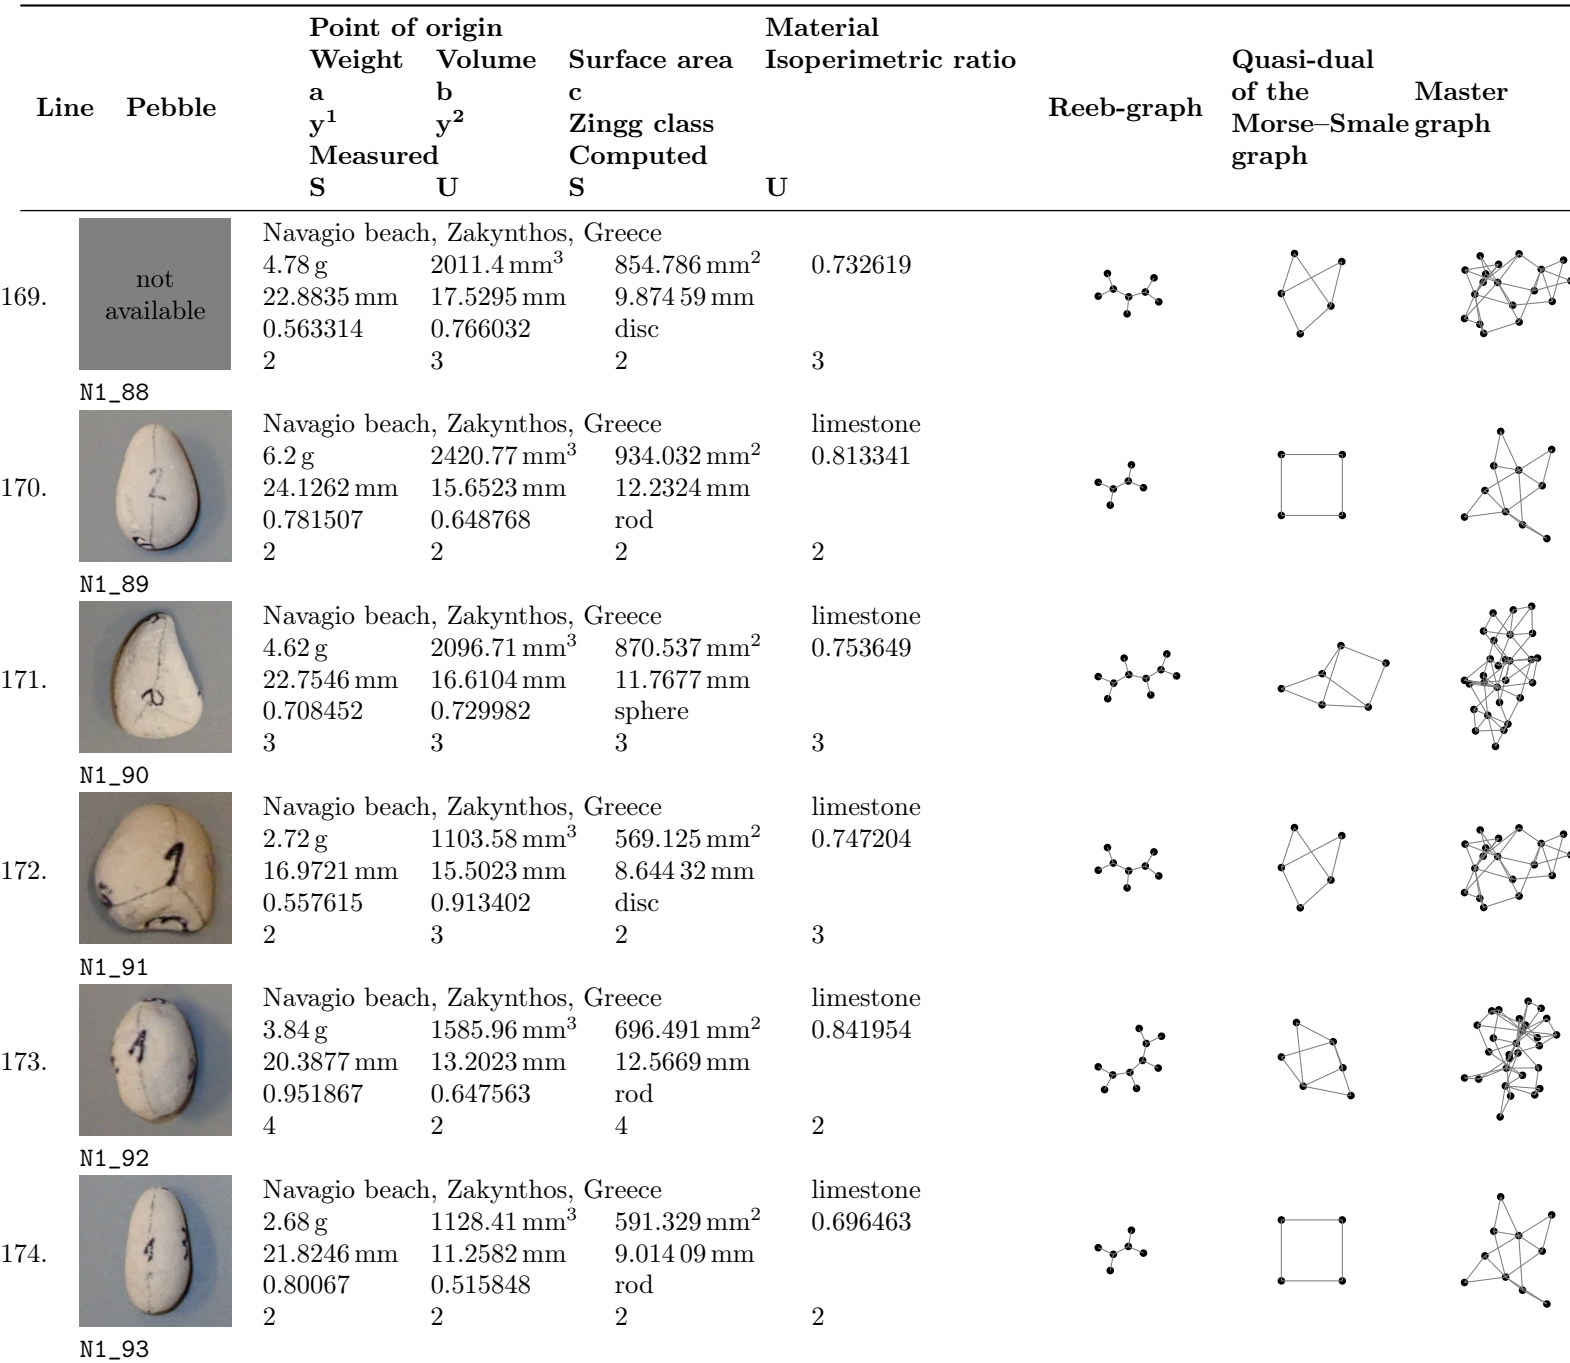   |
|      |                                                                                     | 4.78 g                           | 2011.4 mm <sup>3</sup>  | 854.786 mm <sup>2</sup>      |           |                     |                                                                                       |                                                                                       |                                                                                       |
|      |                                                                                     | 22.8835 mm                       | 17.5295 mm              | 9.874 59 mm                  |           |                     |                                                                                       |                                                                                       |                                                                                       |
|      |                                                                                     | 0.563314                         | 0.766032                | disc                         |           |                     |                                                                                       |                                                                                       |                                                                                       |
|      |                                                                                     | 2                                | 3                       | 2                            |           |                     |                                                                                       |                                                                                       |                                                                                       |
|      | N1_88                                                                               |                                  |                         |                              |           |                     |                                                                                       |                                                                                       |                                                                                       |
| 170. | 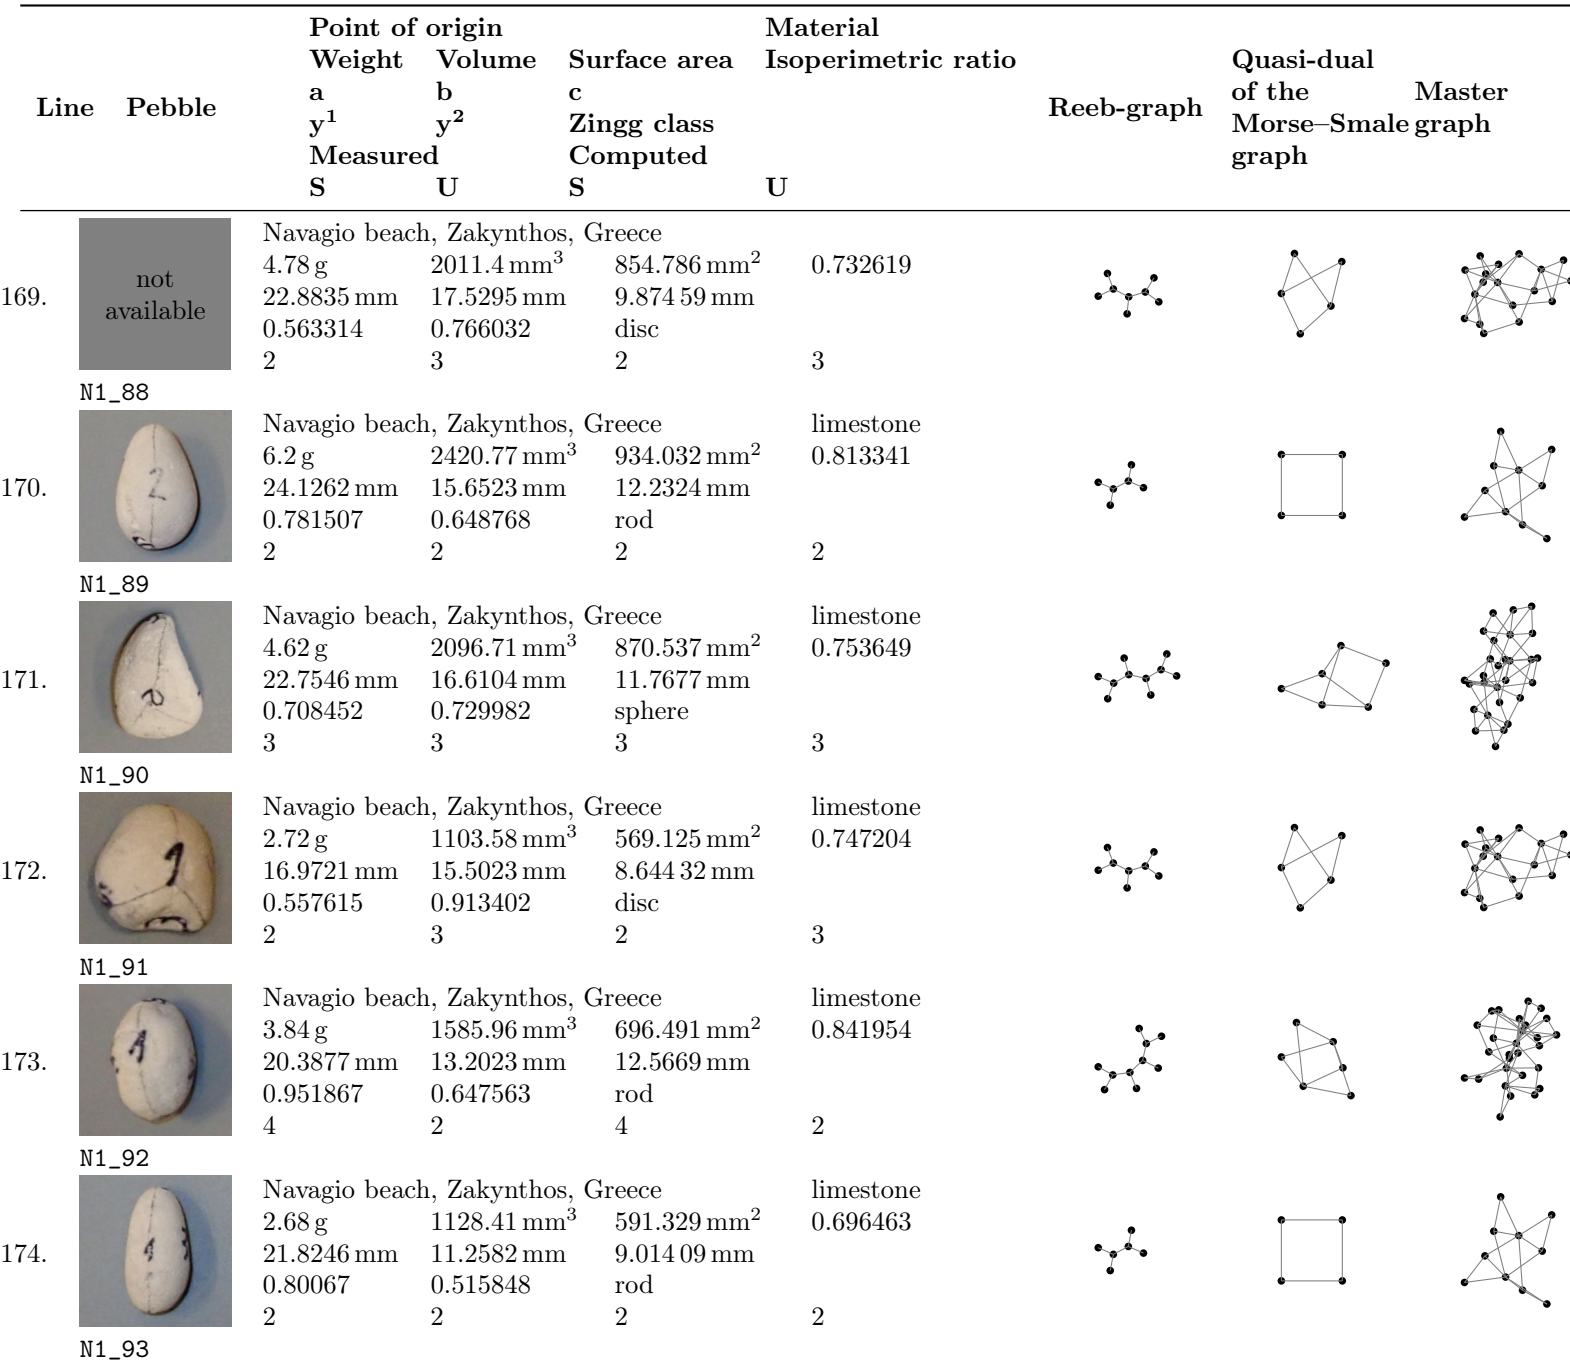   | Navagio beach, Zakynthos, Greece |                         |                              | limestone | 0.813341            | 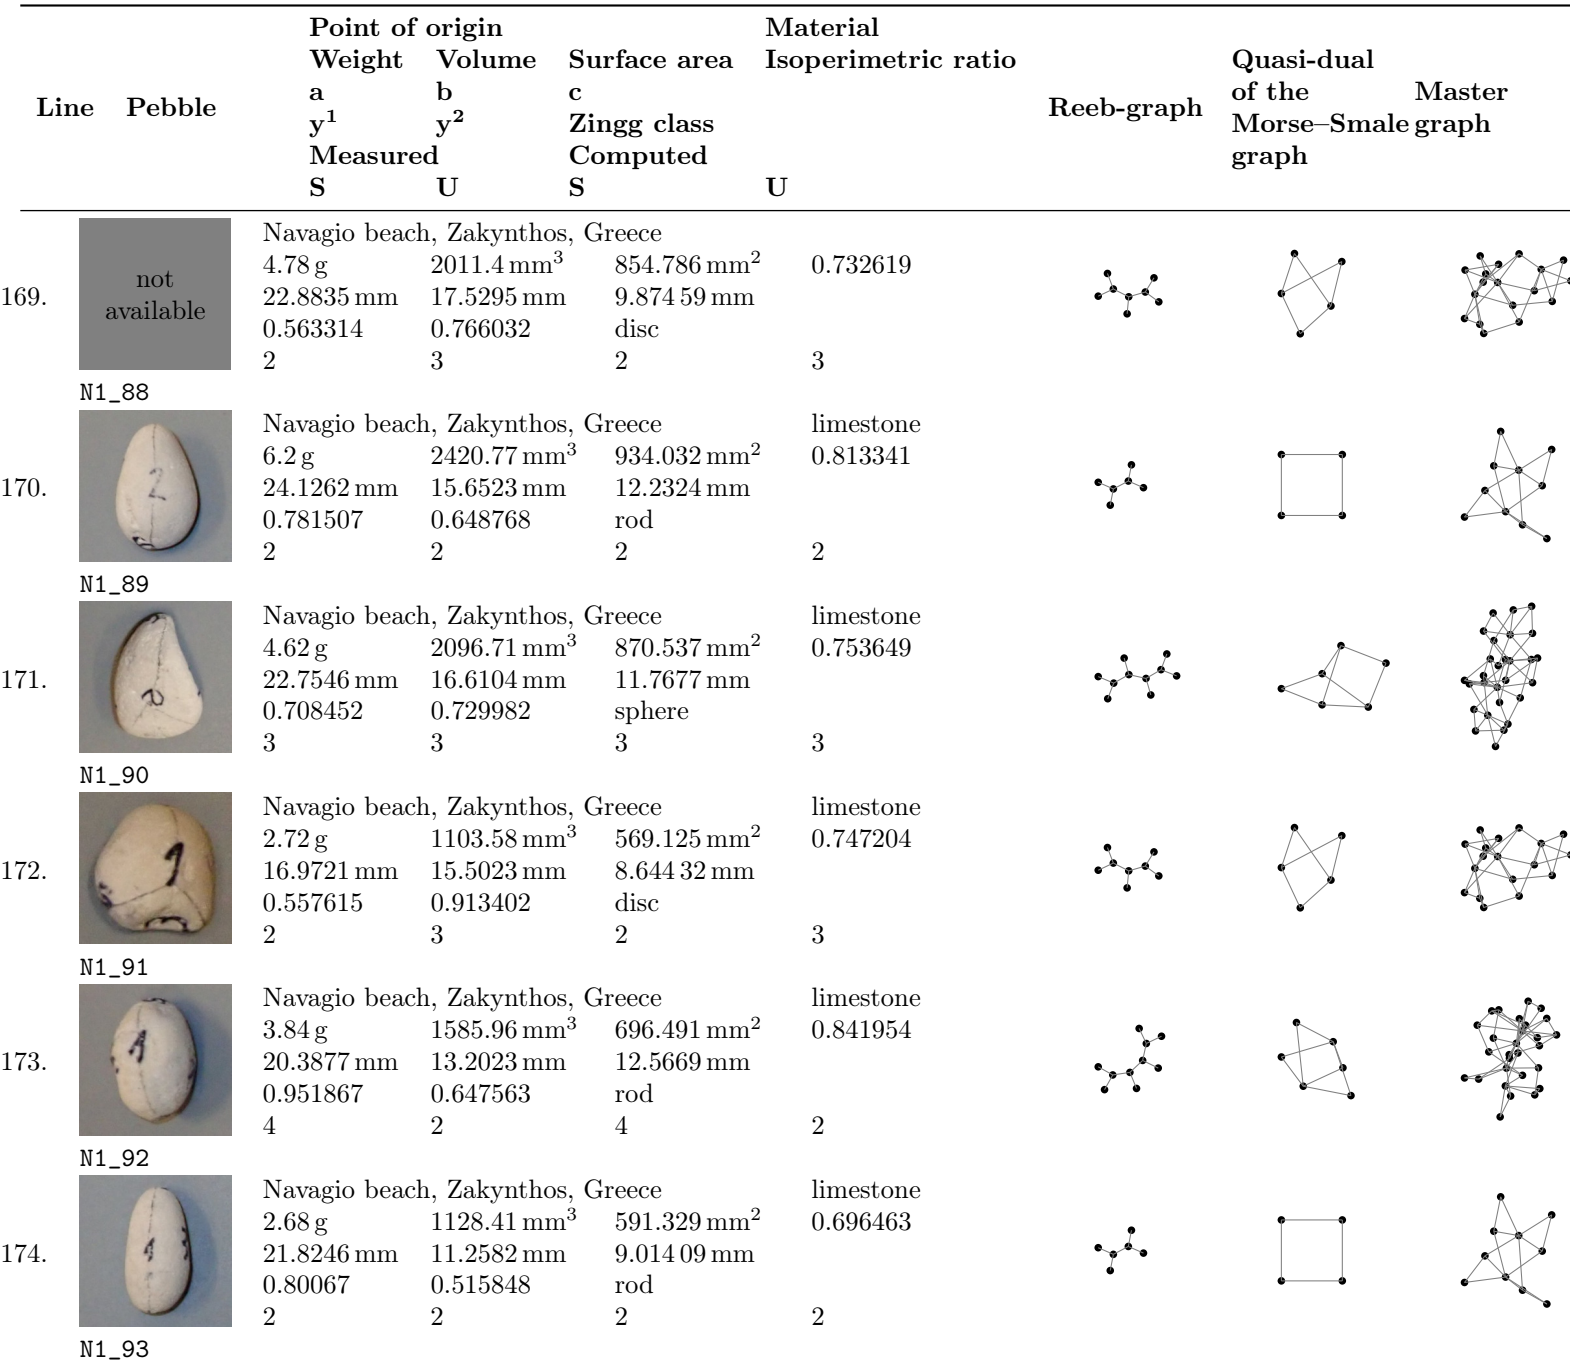   | 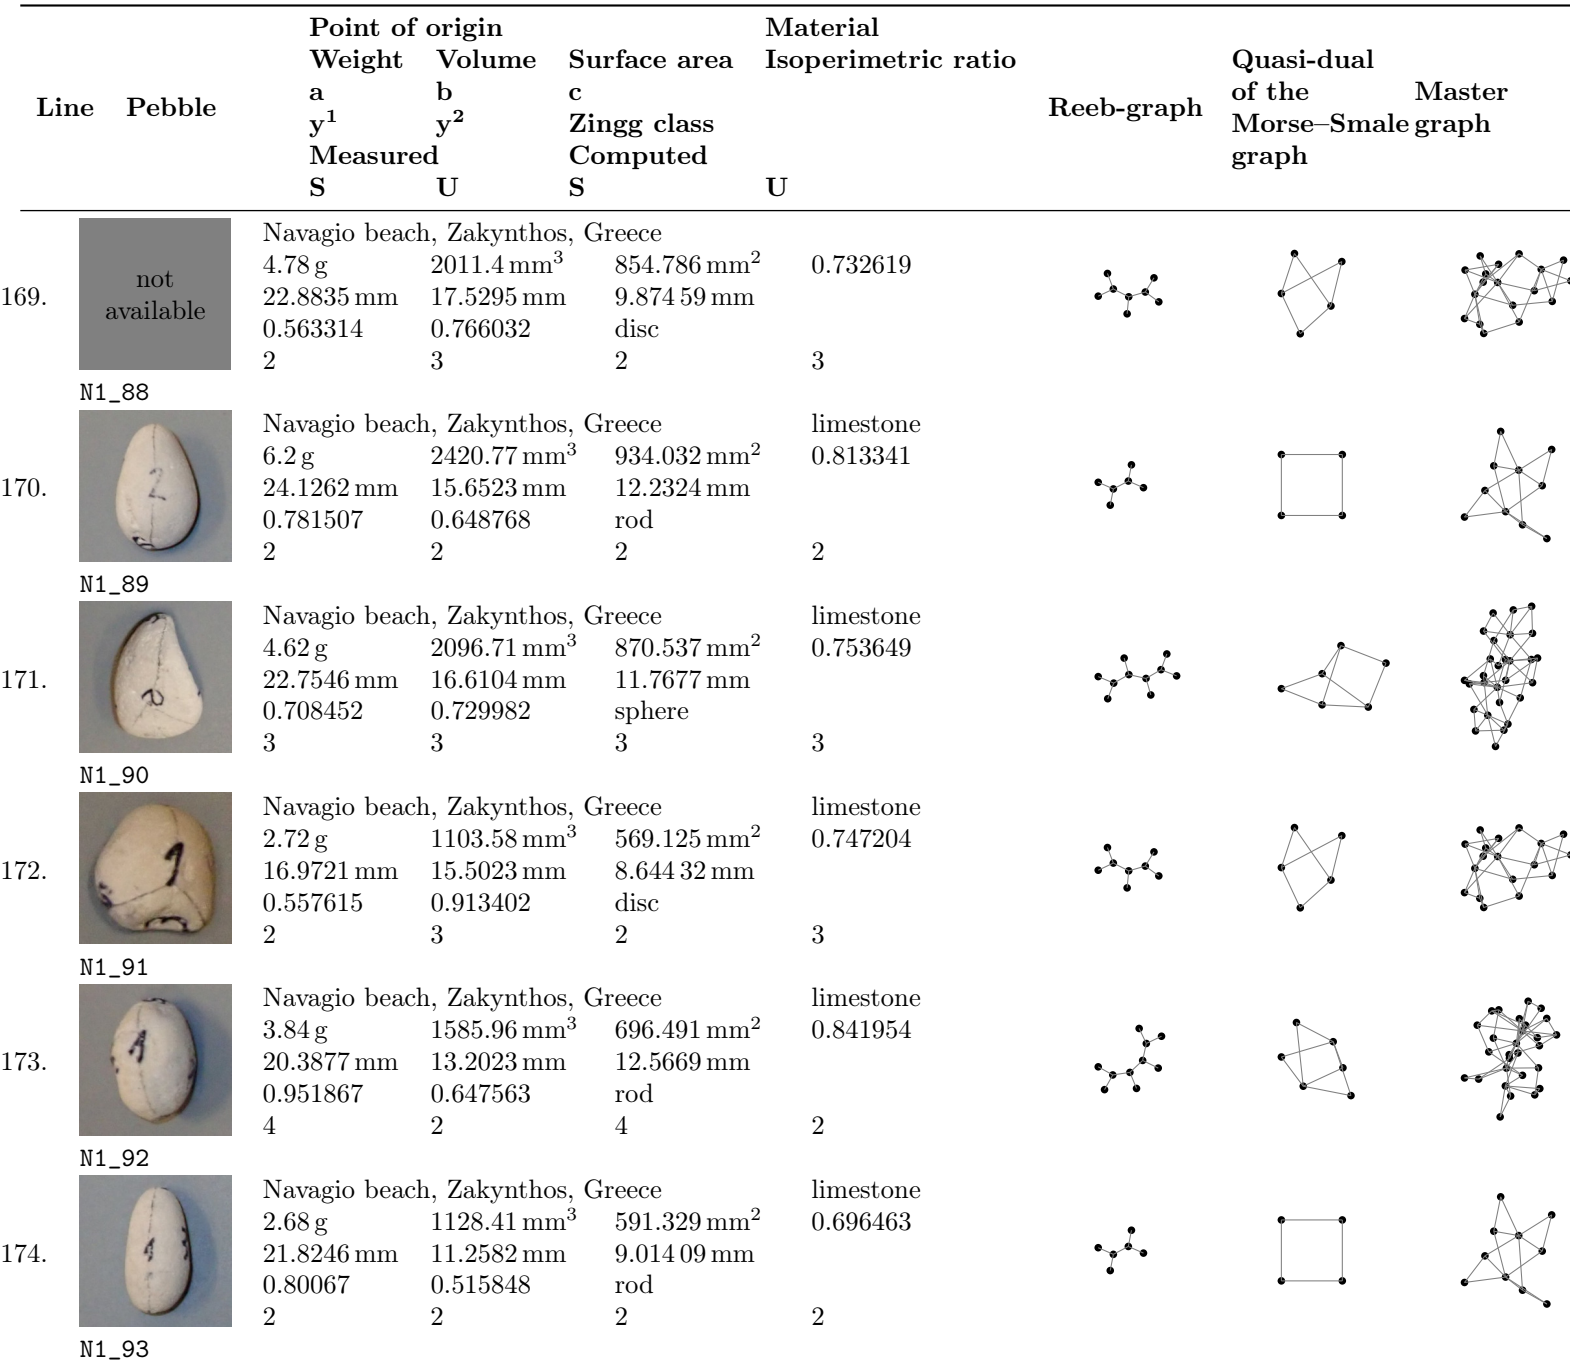   | 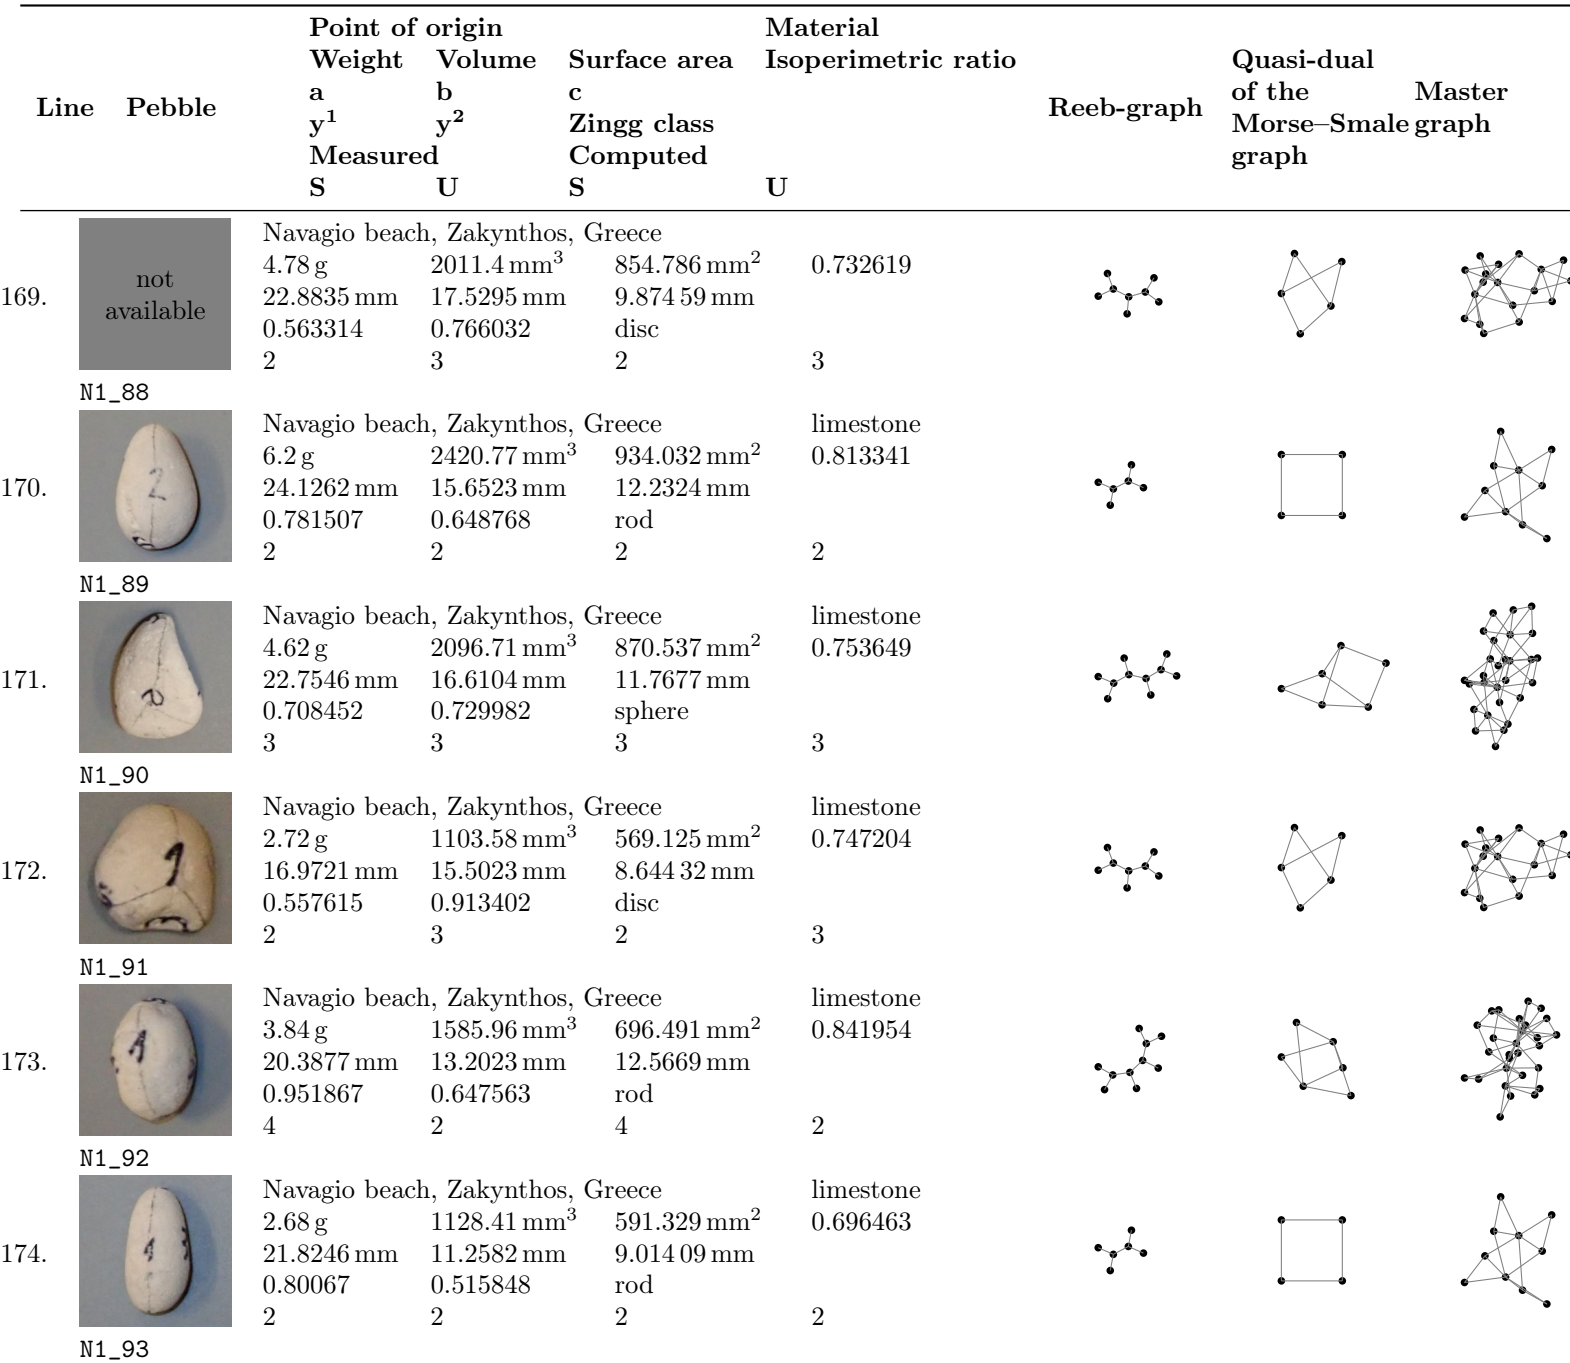   |
|      |                                                                                     | 6.2 g                            | 2420.77 mm <sup>3</sup> | 934.032 mm <sup>2</sup>      |           |                     |                                                                                       |                                                                                       |                                                                                       |
|      |                                                                                     | 24.1262 mm                       | 15.6523 mm              | 12.2324 mm                   |           |                     |                                                                                       |                                                                                       |                                                                                       |
|      |                                                                                     | 0.781507                         | 0.648768                | rod                          |           |                     |                                                                                       |                                                                                       |                                                                                       |
|      |                                                                                     | 2                                | 2                       | 2                            |           |                     |                                                                                       |                                                                                       |                                                                                       |
|      | N1_89                                                                               |                                  |                         |                              |           |                     |                                                                                       |                                                                                       |                                                                                       |
| 171. | 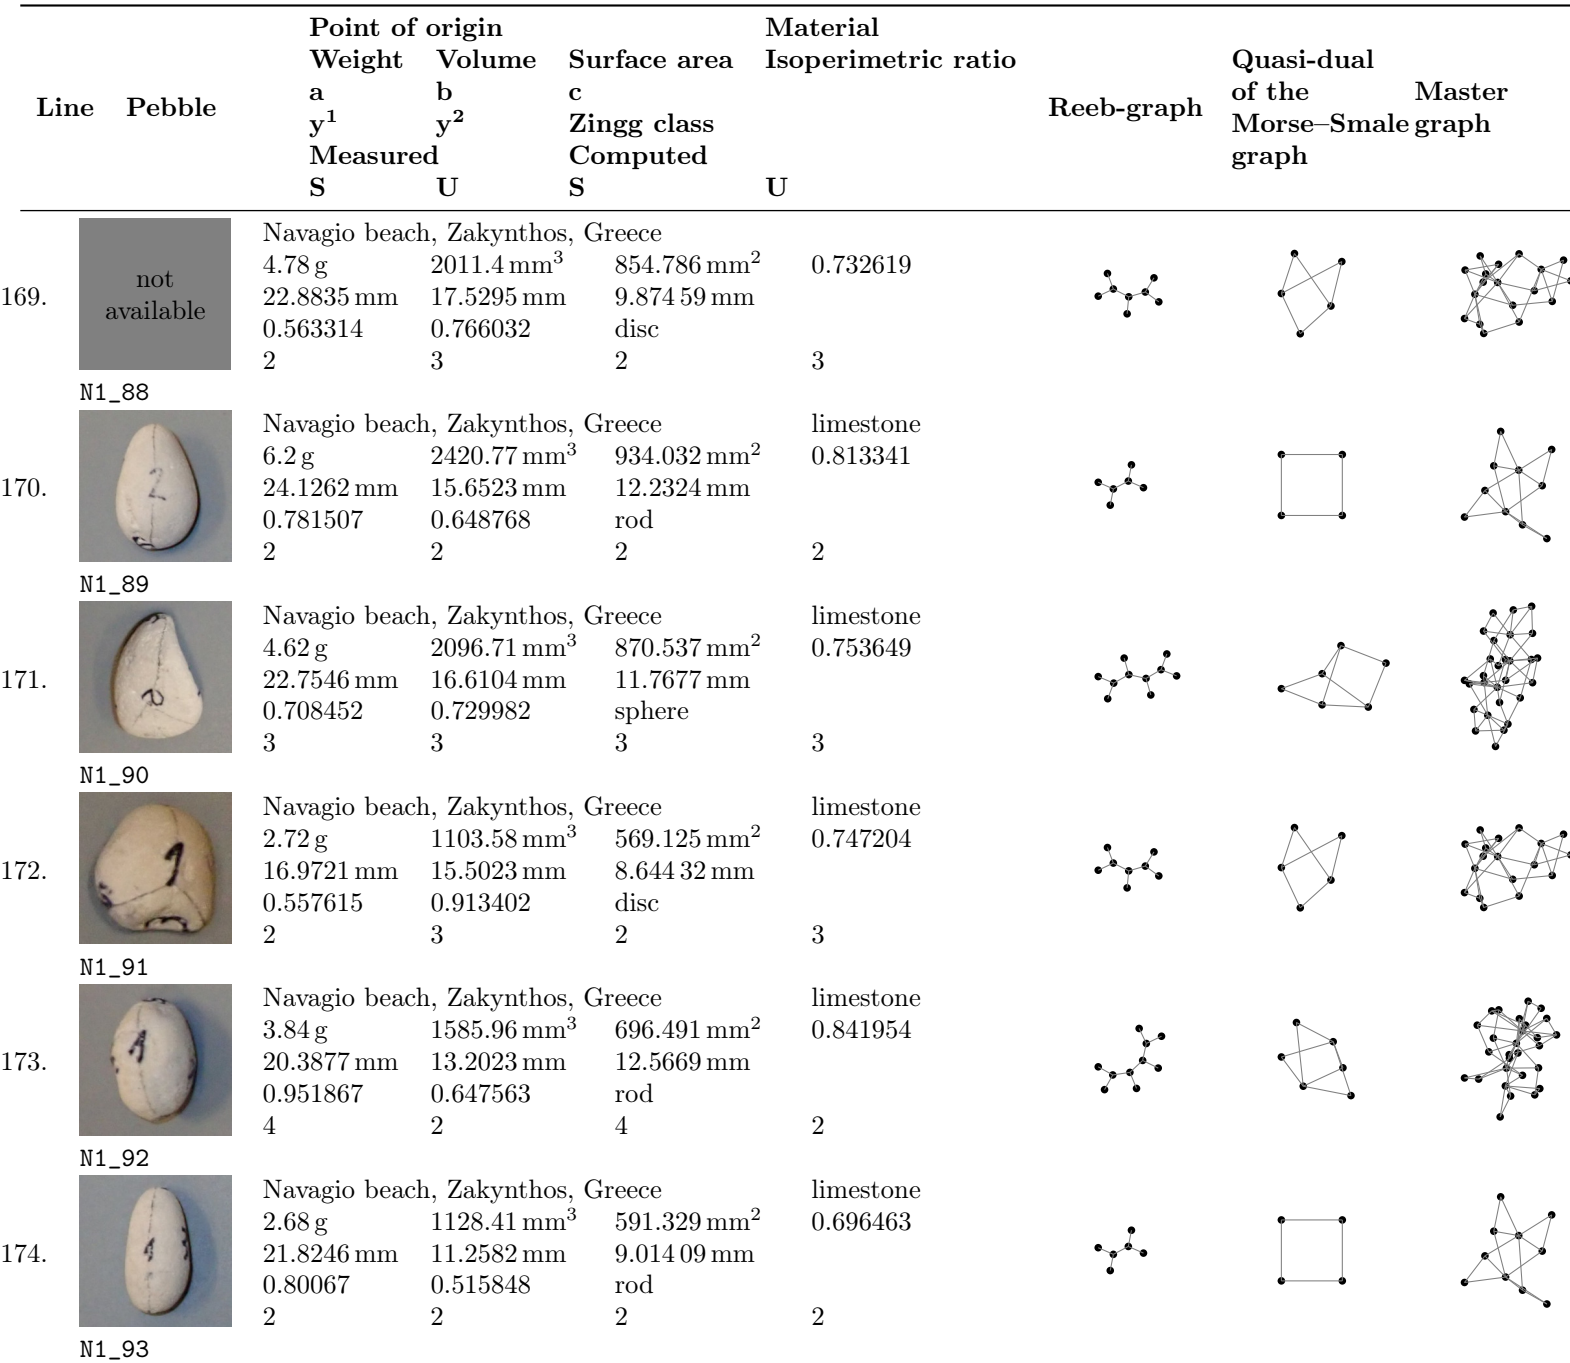   | Navagio beach, Zakynthos, Greece |                         |                              | limestone | 0.753649            | 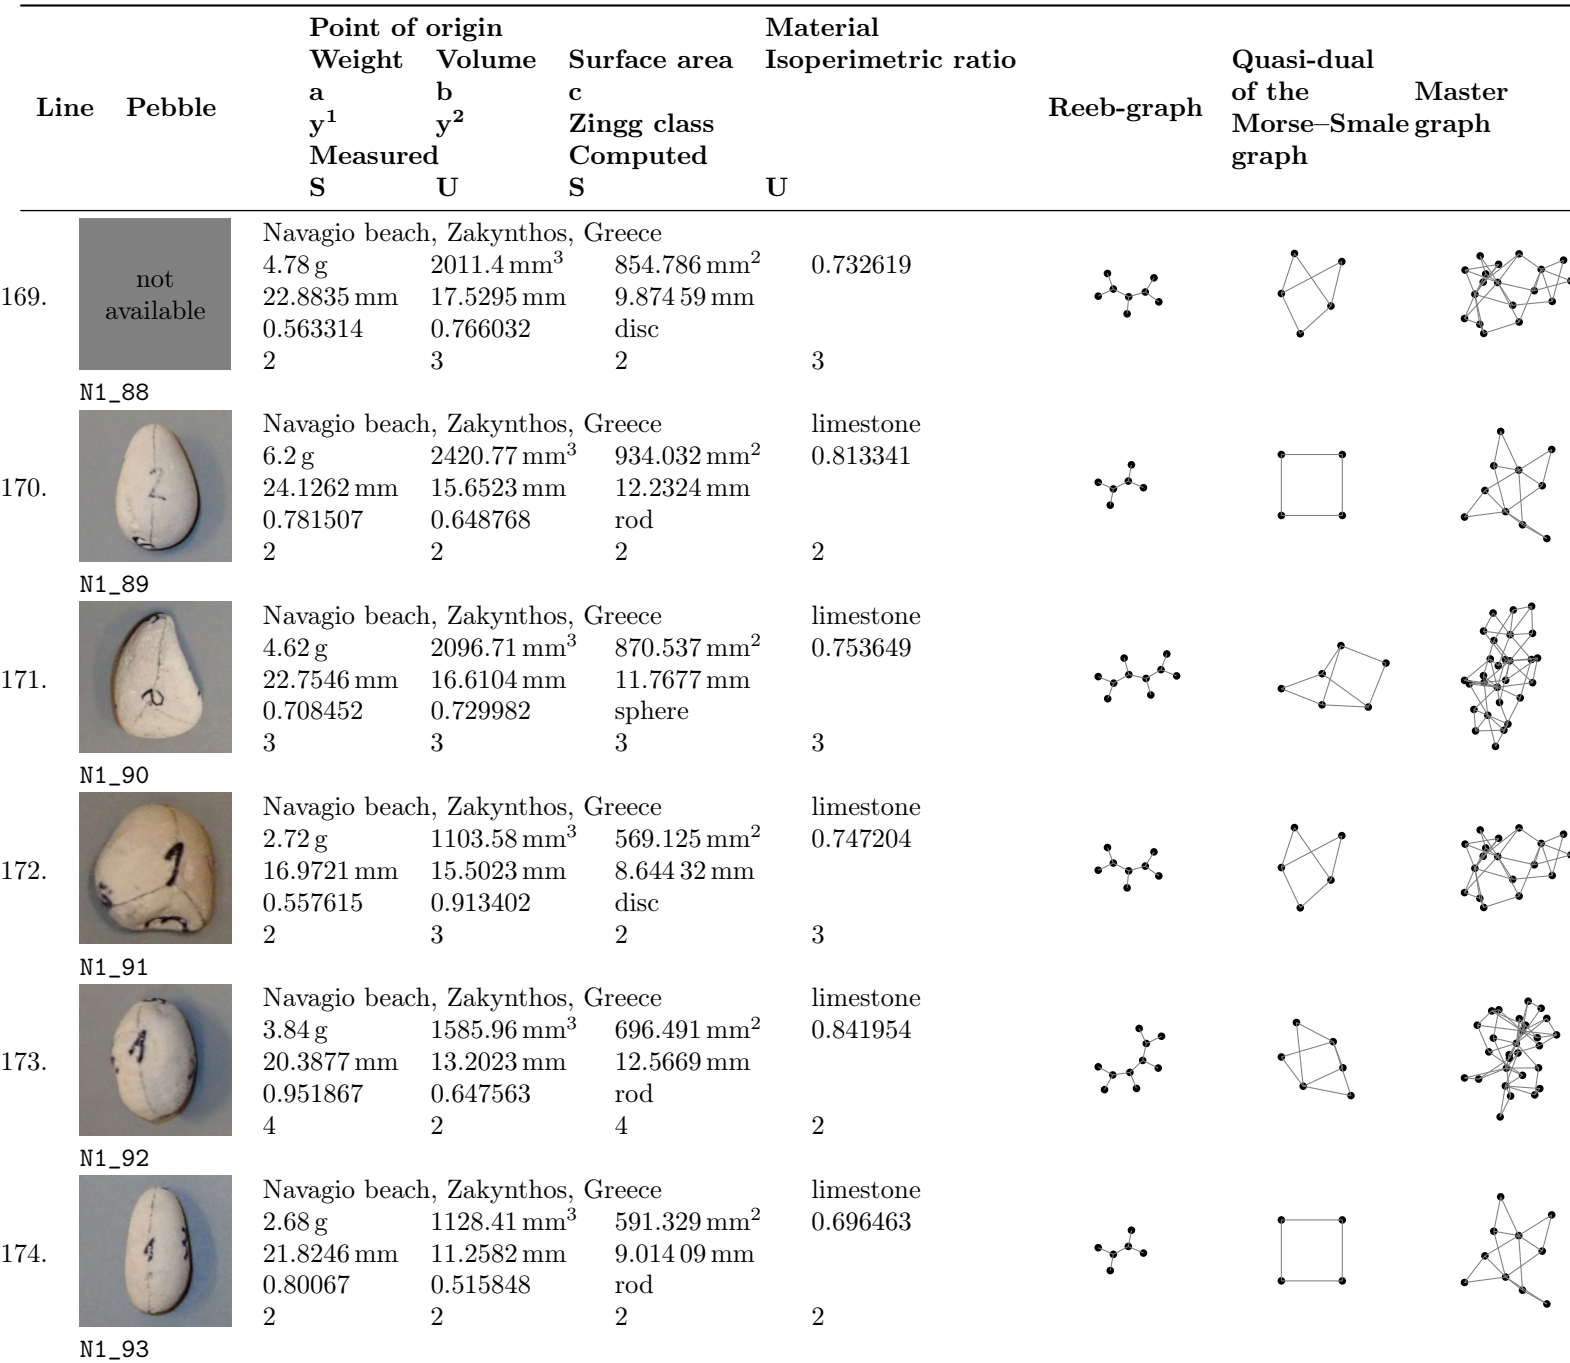   | 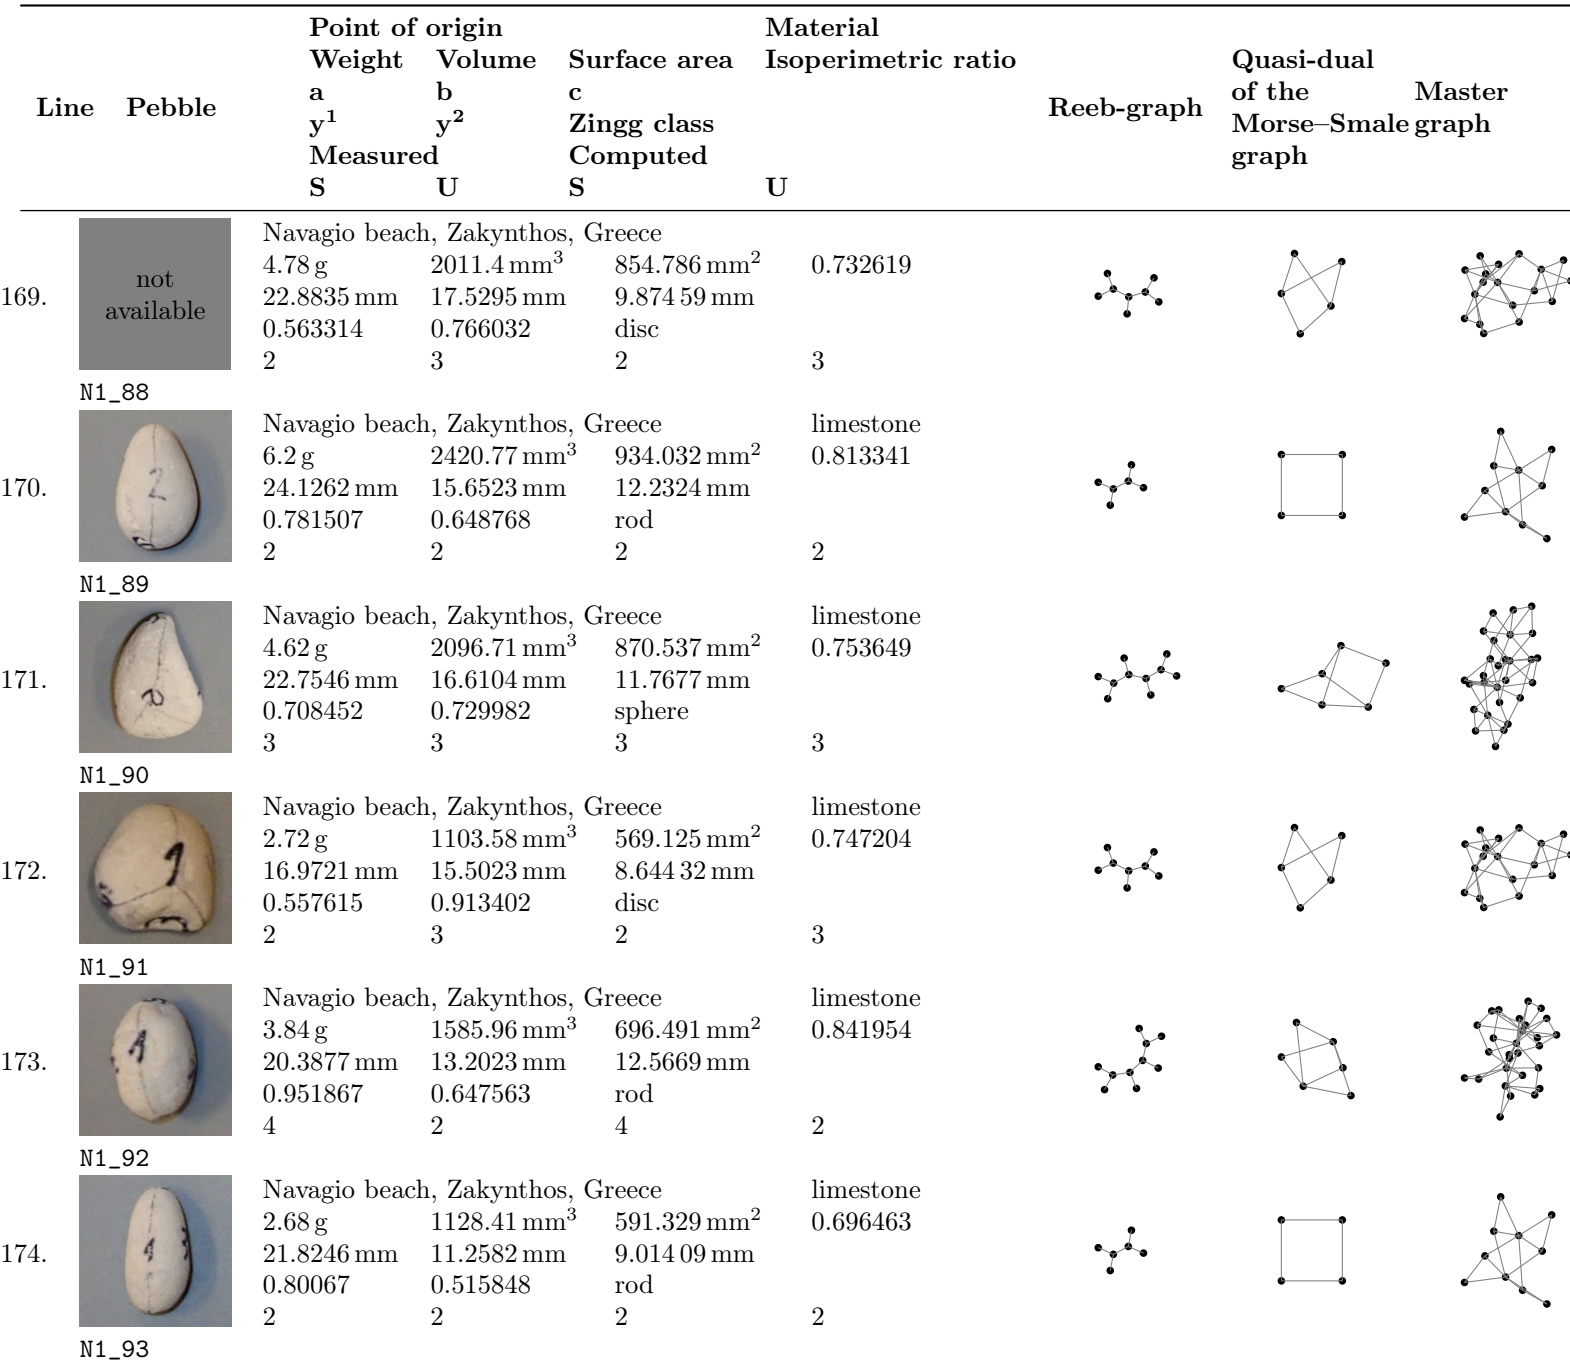   | 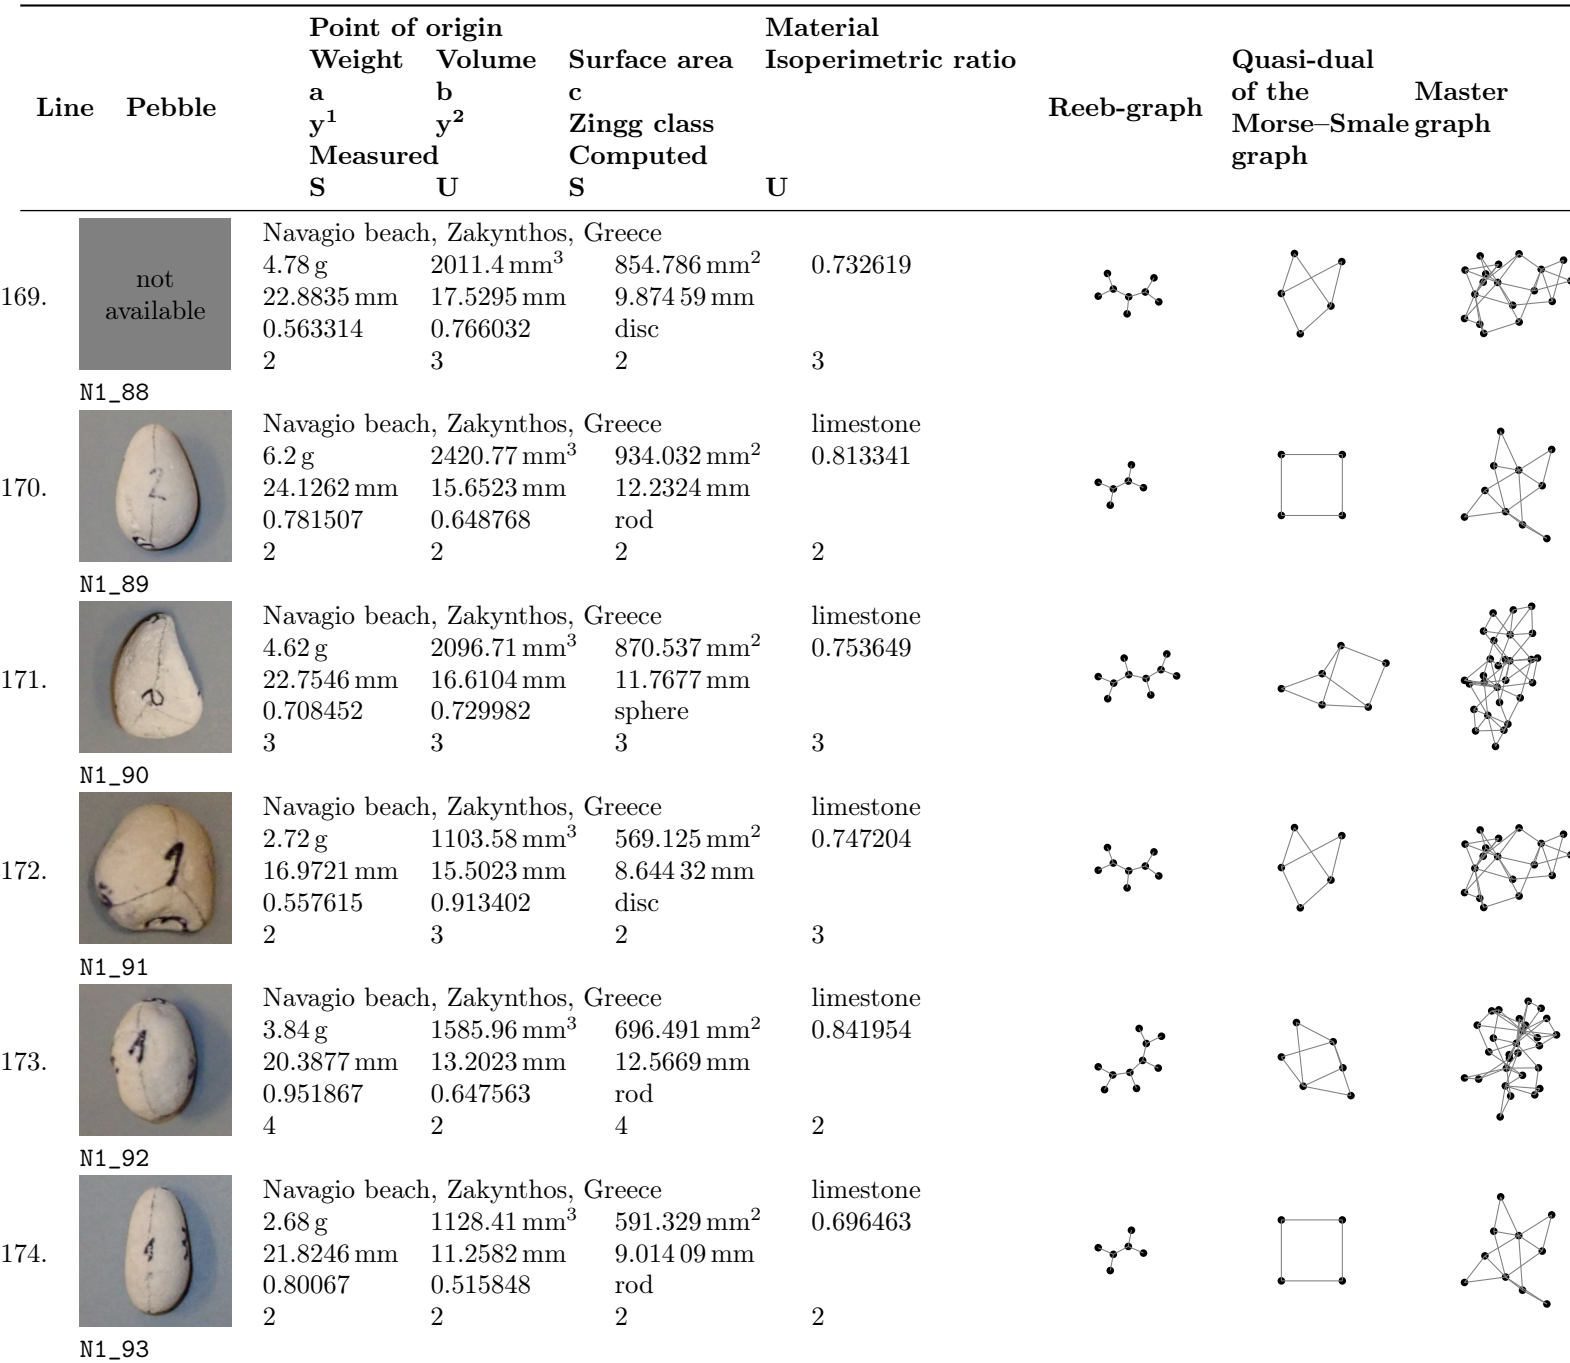   |
|      |                                                                                     | 4.62 g                           | 2096.71 mm <sup>3</sup> | 870.537 mm <sup>2</sup>      |           |                     |                                                                                       |                                                                                       |                                                                                       |
|      |                                                                                     | 22.7546 mm                       | 16.6104 mm              | 11.7677 mm                   |           |                     |                                                                                       |                                                                                       |                                                                                       |
|      |                                                                                     | 0.708452                         | 0.729982                | sphere                       |           |                     |                                                                                       |                                                                                       |                                                                                       |
|      |                                                                                     | 3                                | 3                       | 3                            |           |                     |                                                                                       |                                                                                       |                                                                                       |
|      | N1_90                                                                               |                                  |                         |                              |           |                     |                                                                                       |                                                                                       |                                                                                       |
| 172. | 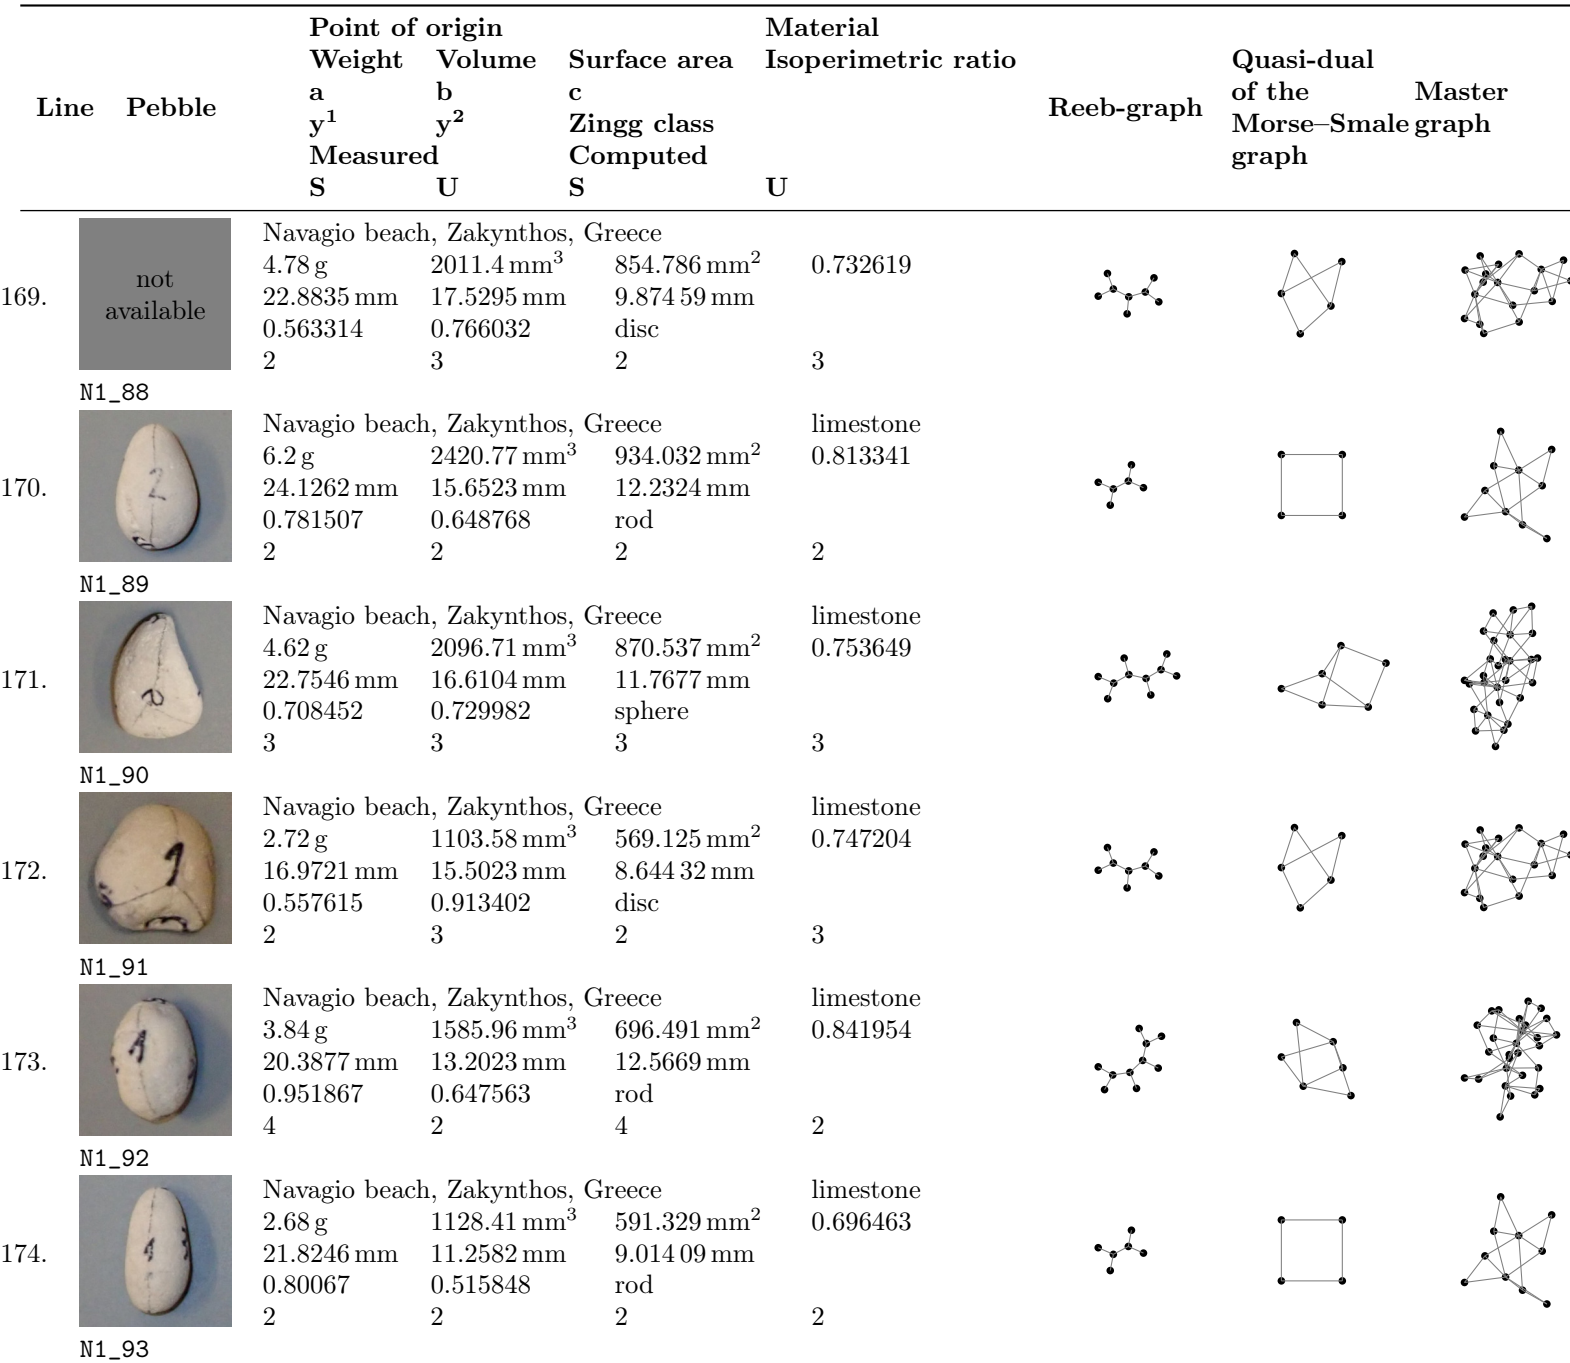  | Navagio beach, Zakynthos, Greece |                         |                              | limestone | 0.747204            | 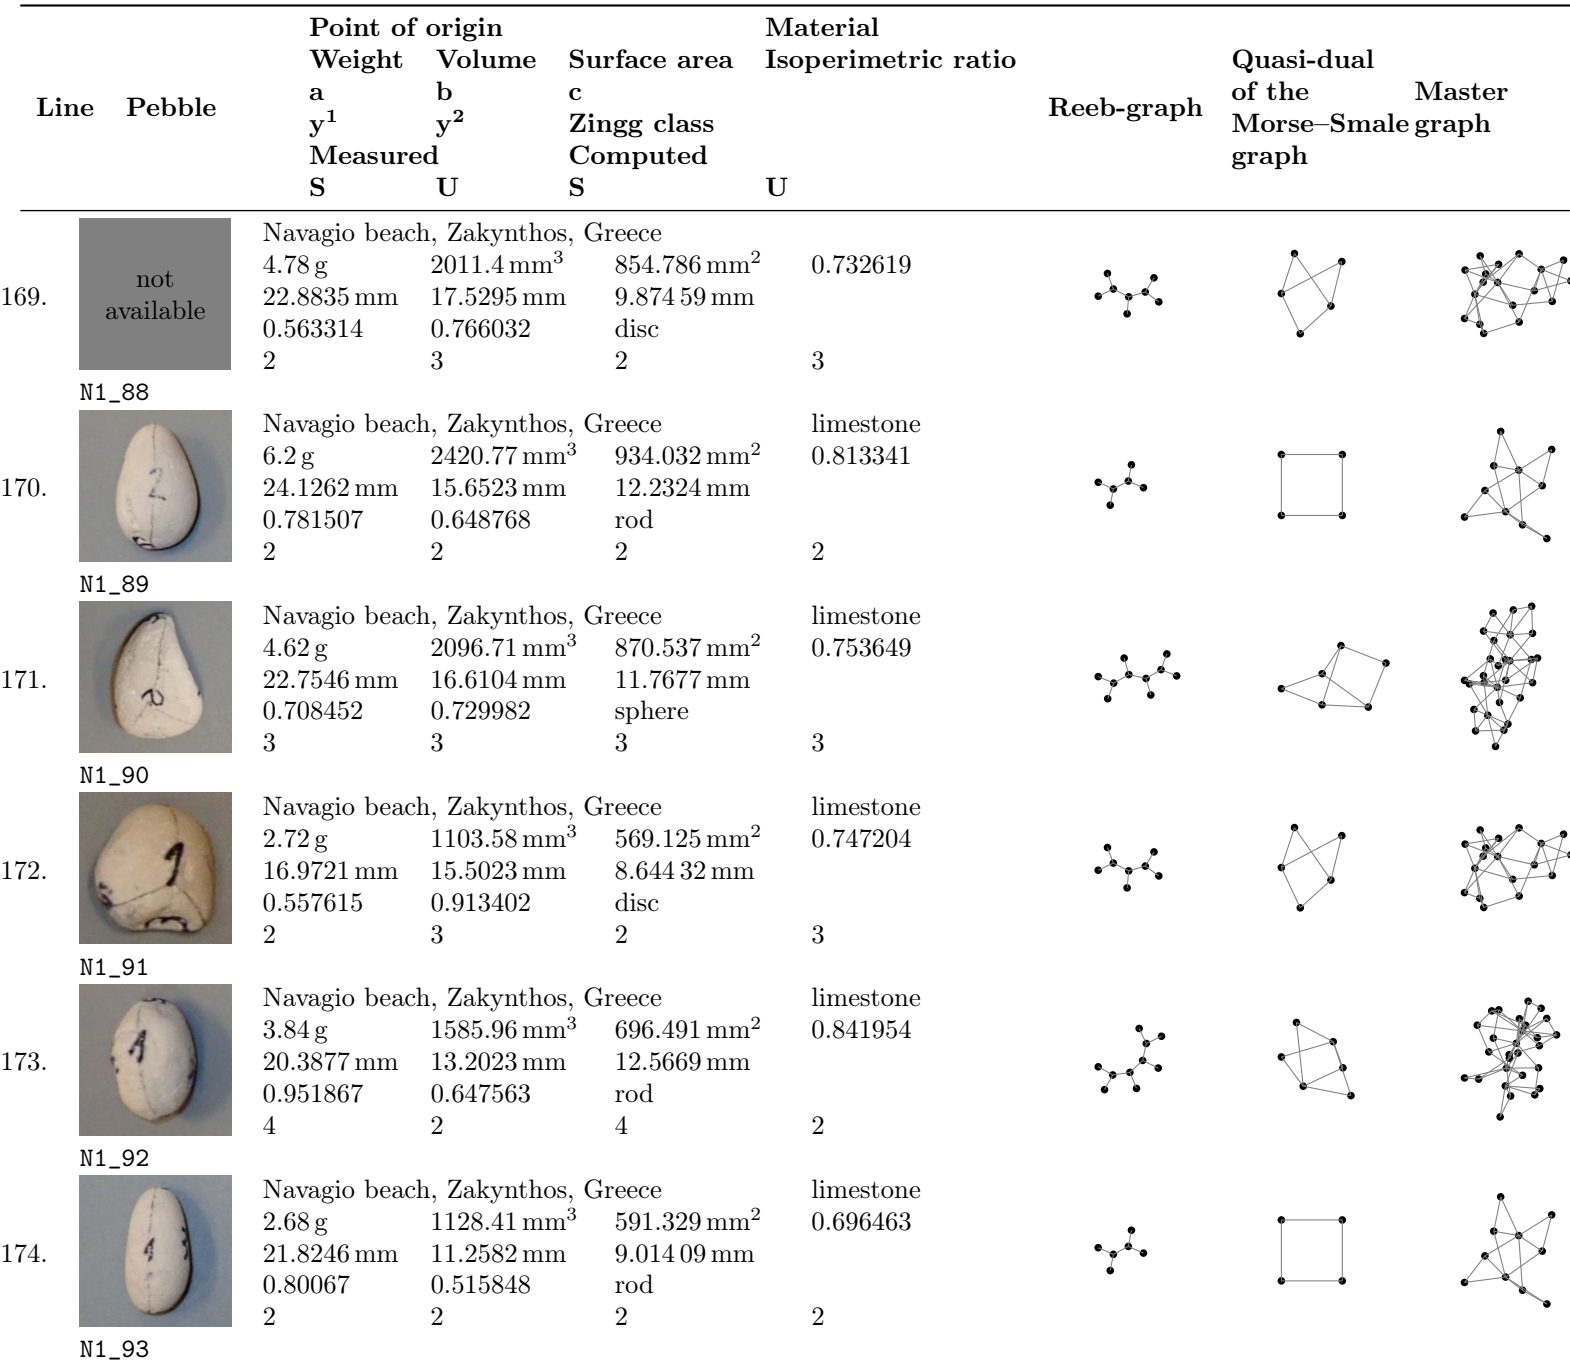  | 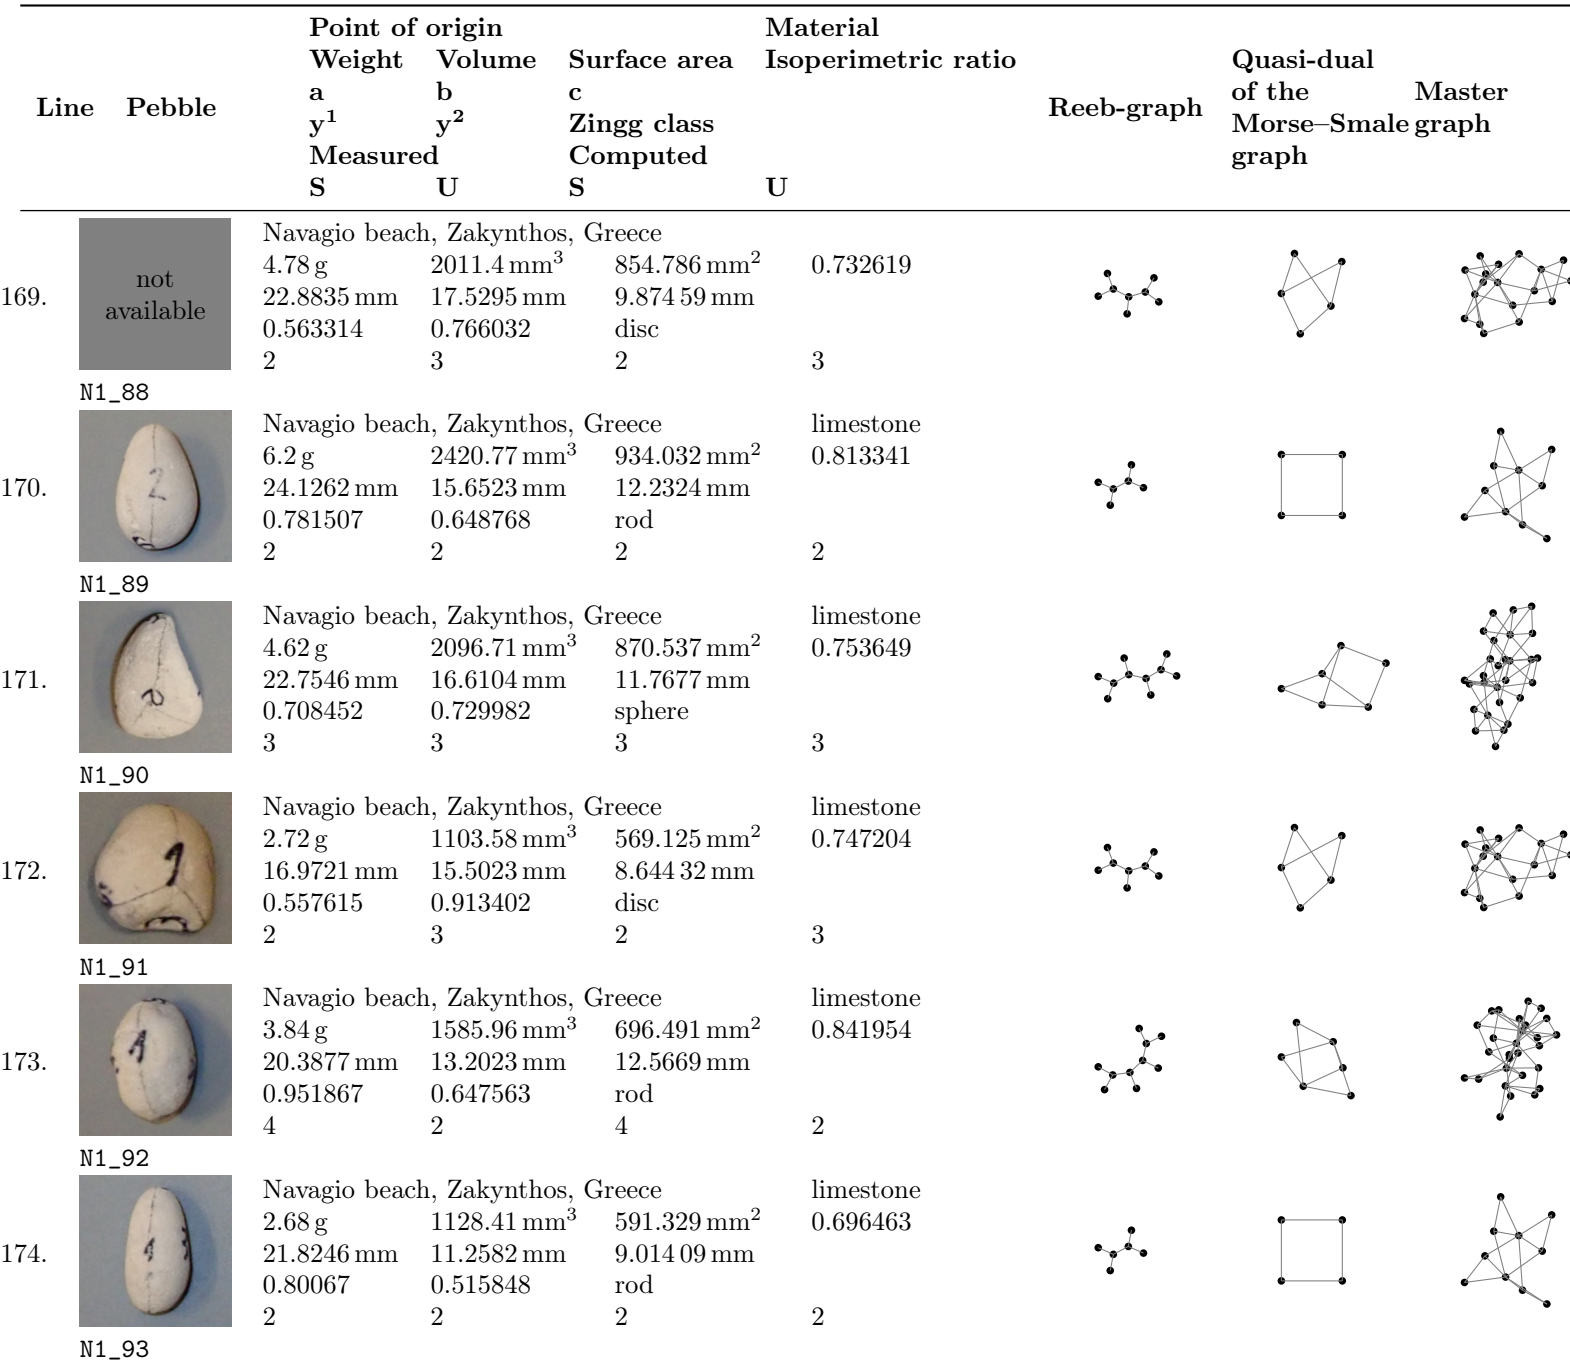  | 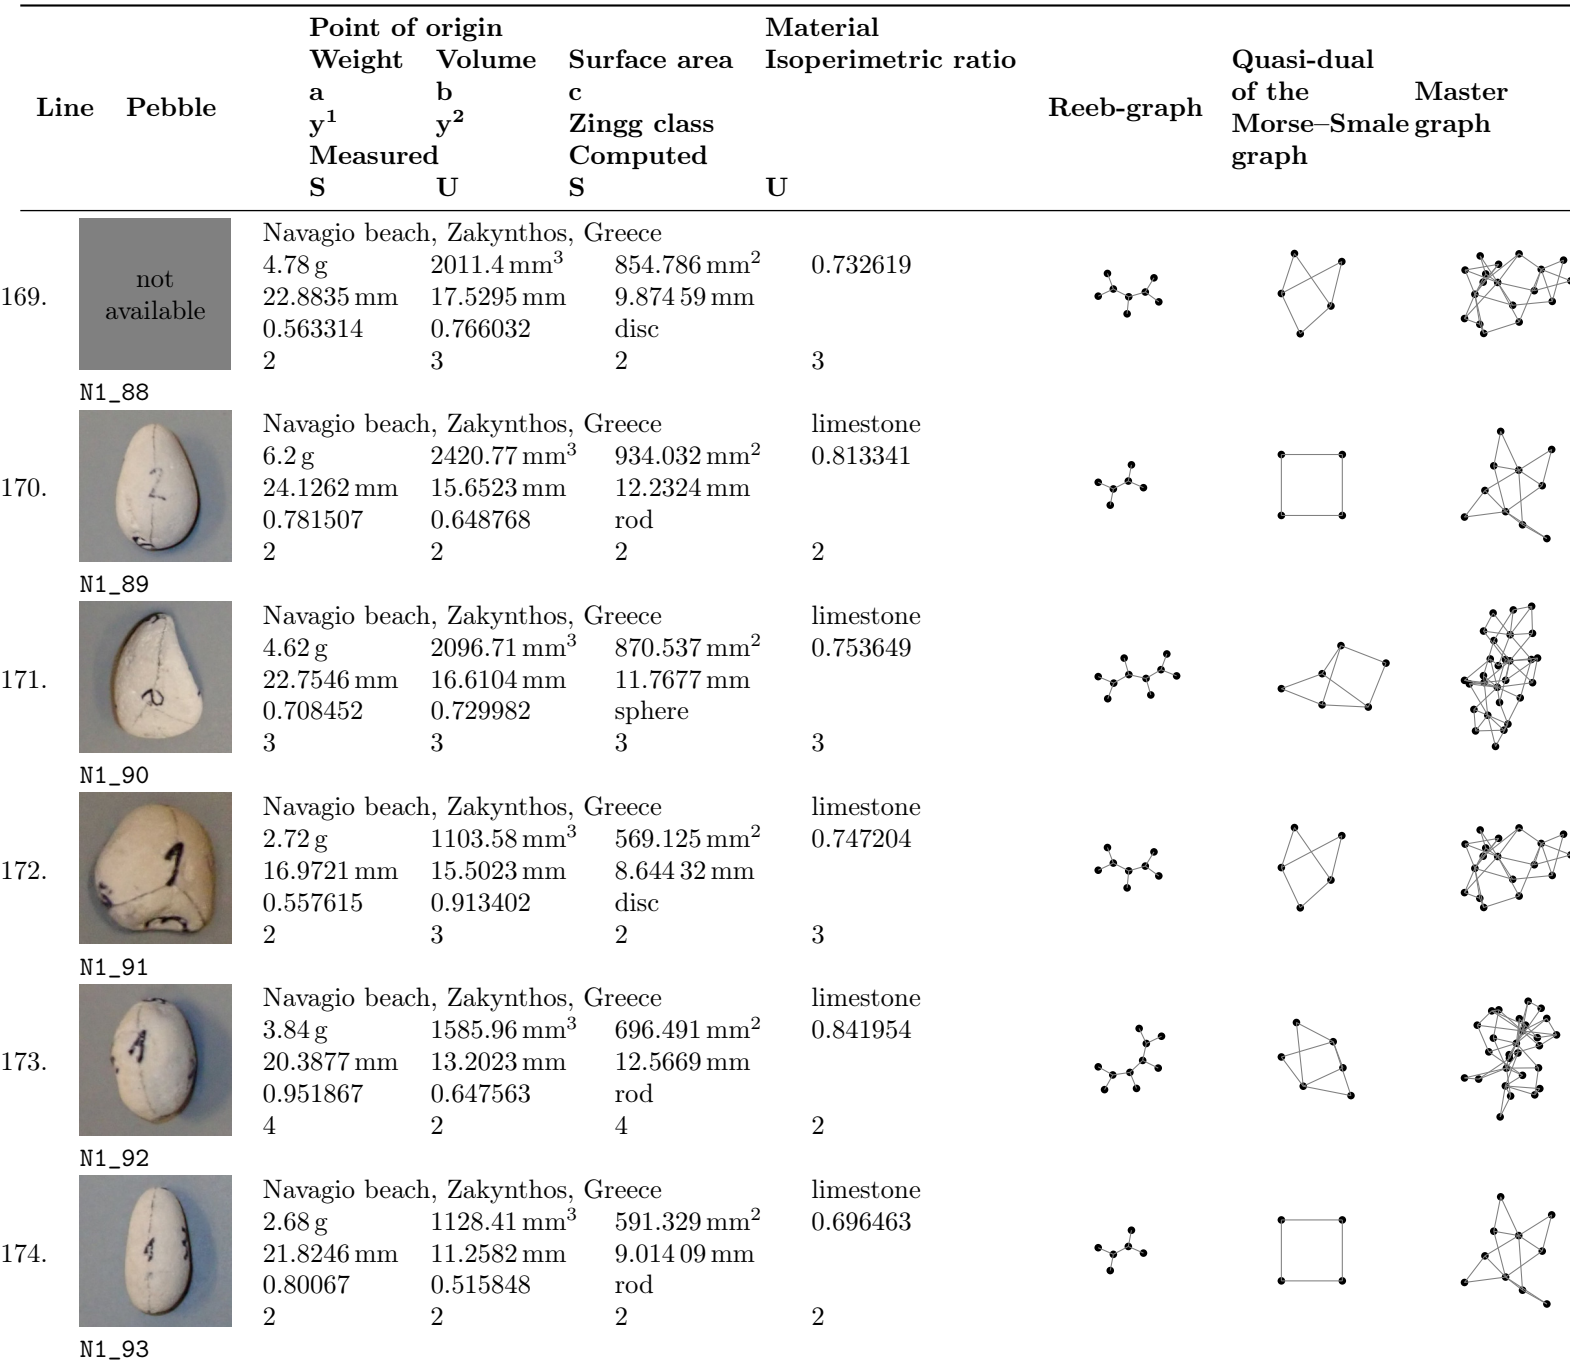  |
|      |                                                                                     | 2.72 g                           | 1103.58 mm <sup>3</sup> | 569.125 mm <sup>2</sup>      |           |                     |                                                                                       |                                                                                       |                                                                                       |
|      |                                                                                     | 16.9721 mm                       | 15.5023 mm              | 8.644 32 mm                  |           |                     |                                                                                       |                                                                                       |                                                                                       |
|      |                                                                                     | 0.557615                         | 0.913402                | disc                         |           |                     |                                                                                       |                                                                                       |                                                                                       |
|      |                                                                                     | 2                                | 3                       | 2                            |           |                     |                                                                                       |                                                                                       |                                                                                       |
|      | N1_91                                                                               |                                  |                         |                              |           |                     |                                                                                       |                                                                                       |                                                                                       |
| 173. | 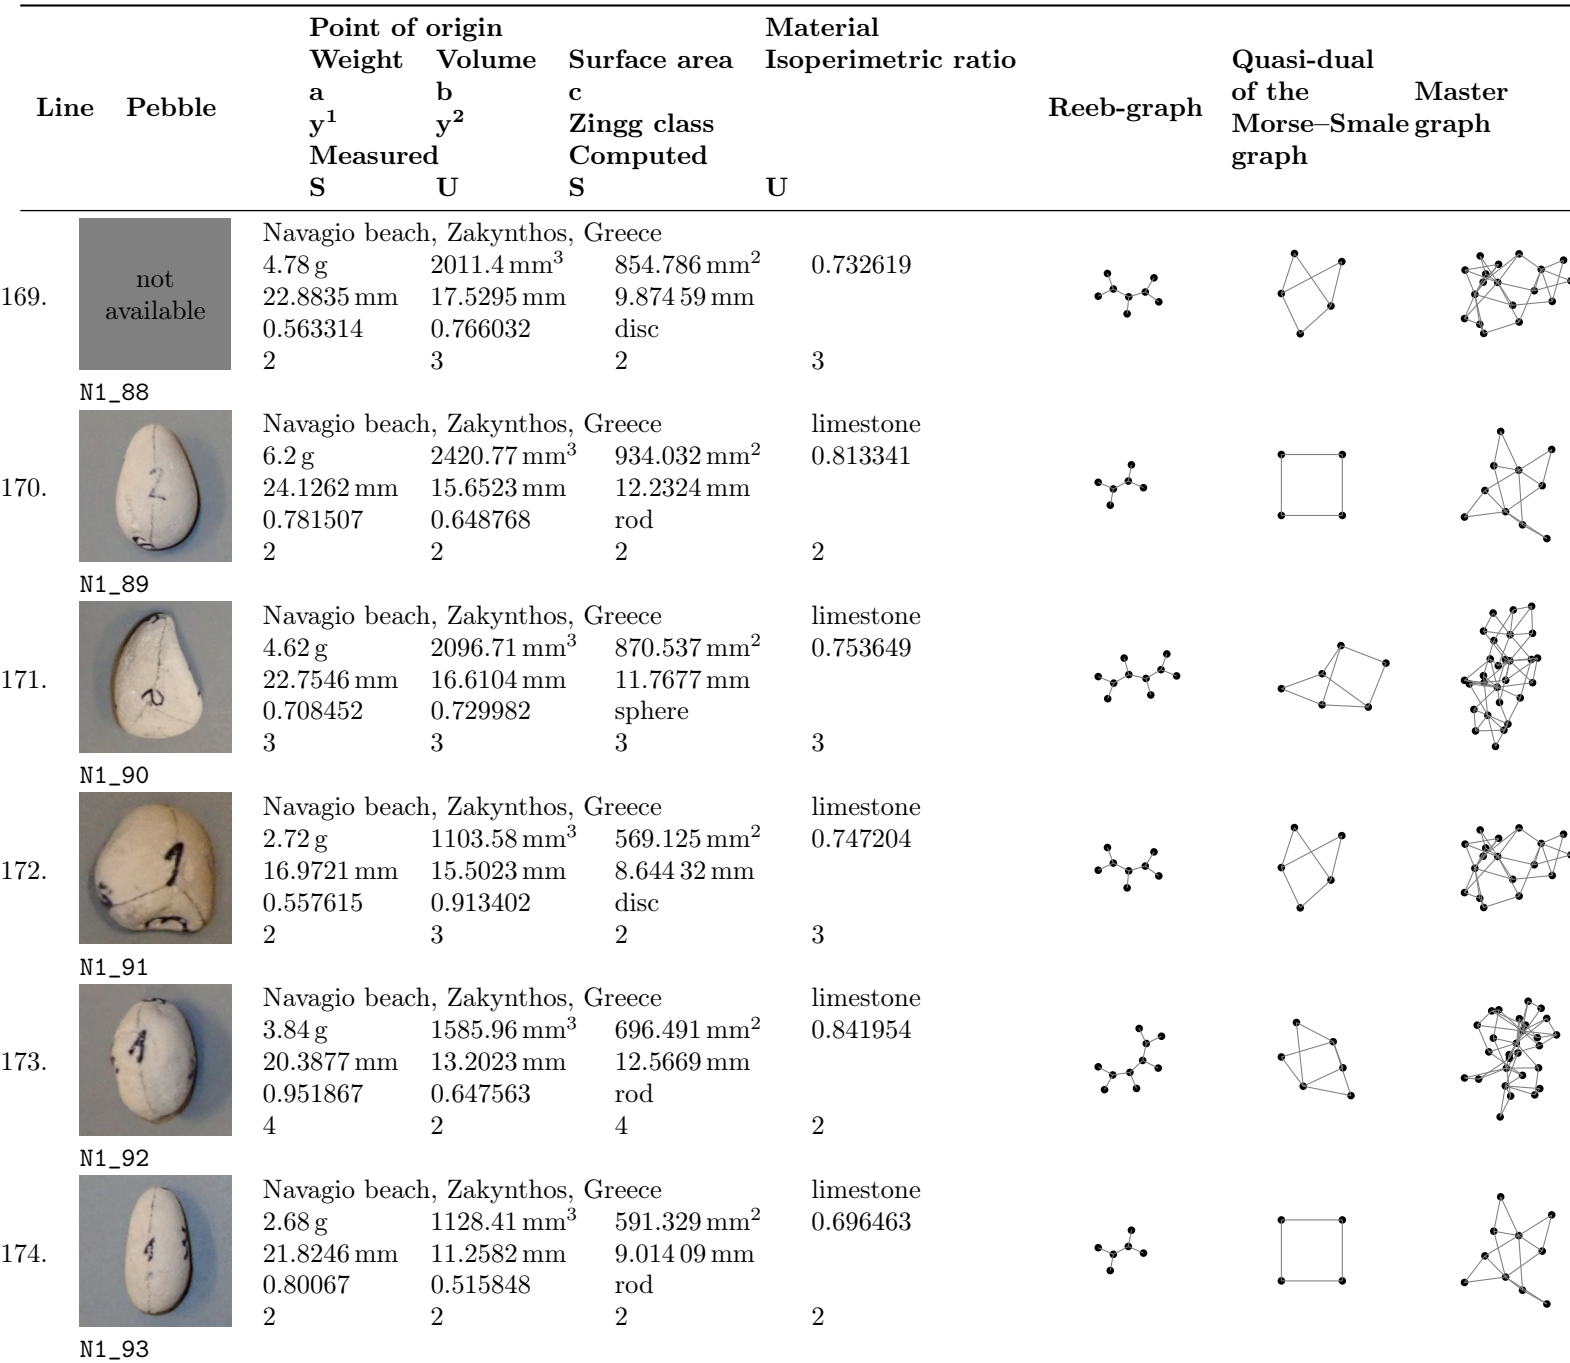 | Navagio beach, Zakynthos, Greece |                         |                              | limestone | 0.841954            | 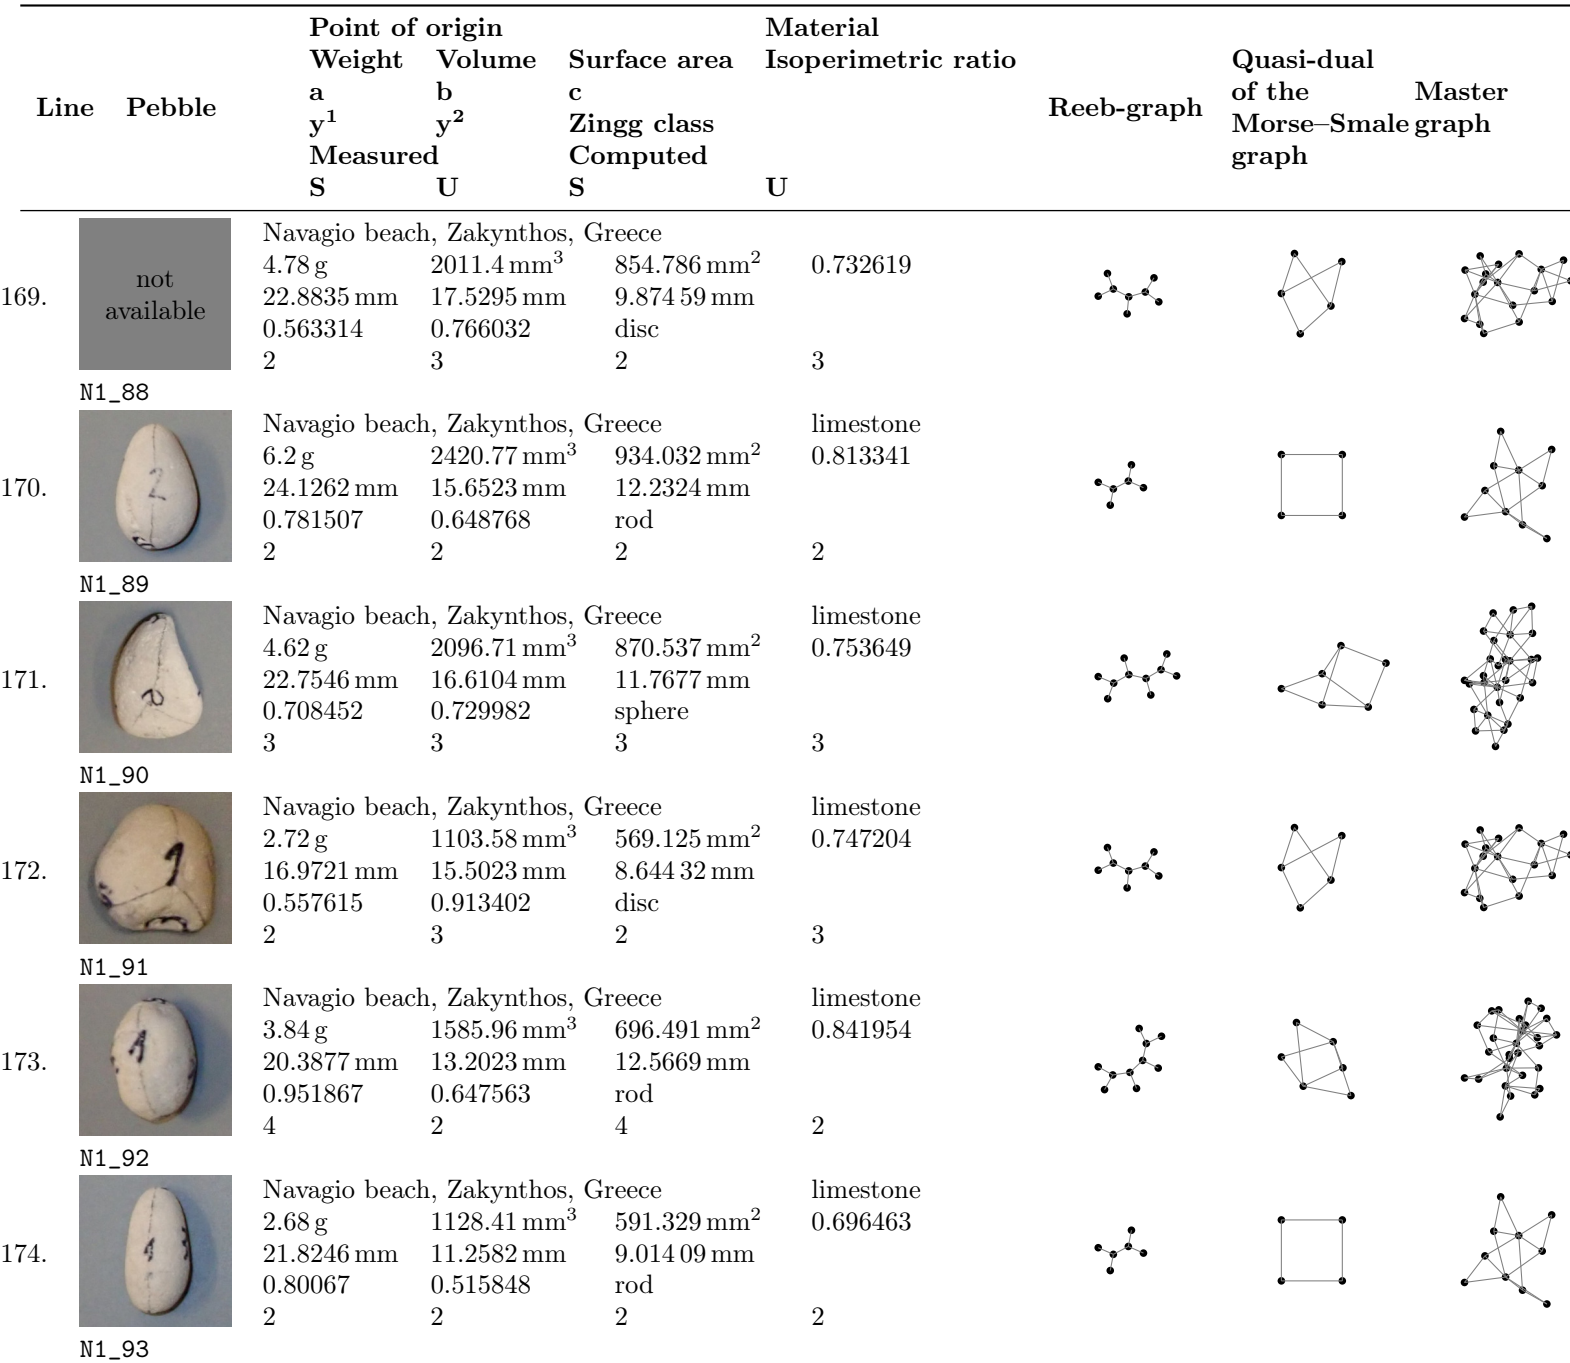 | 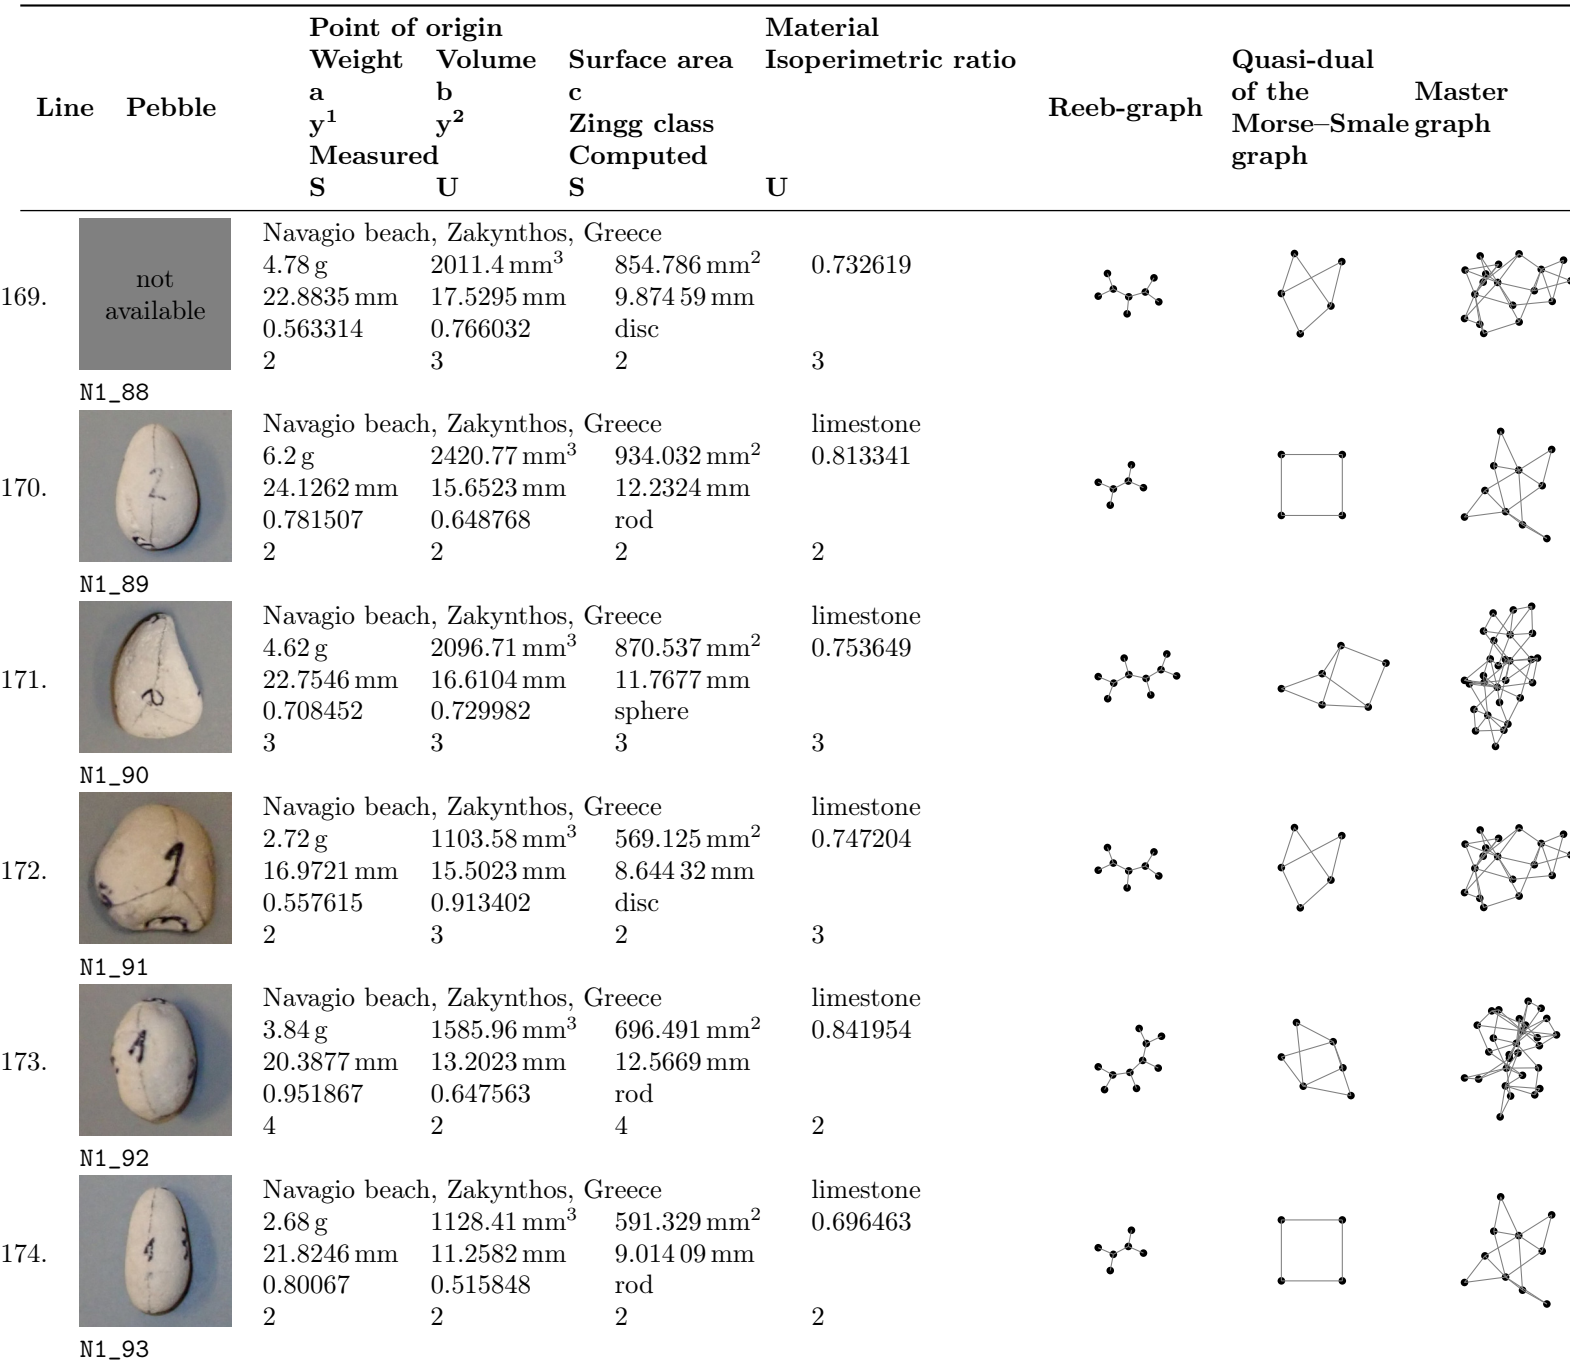 | 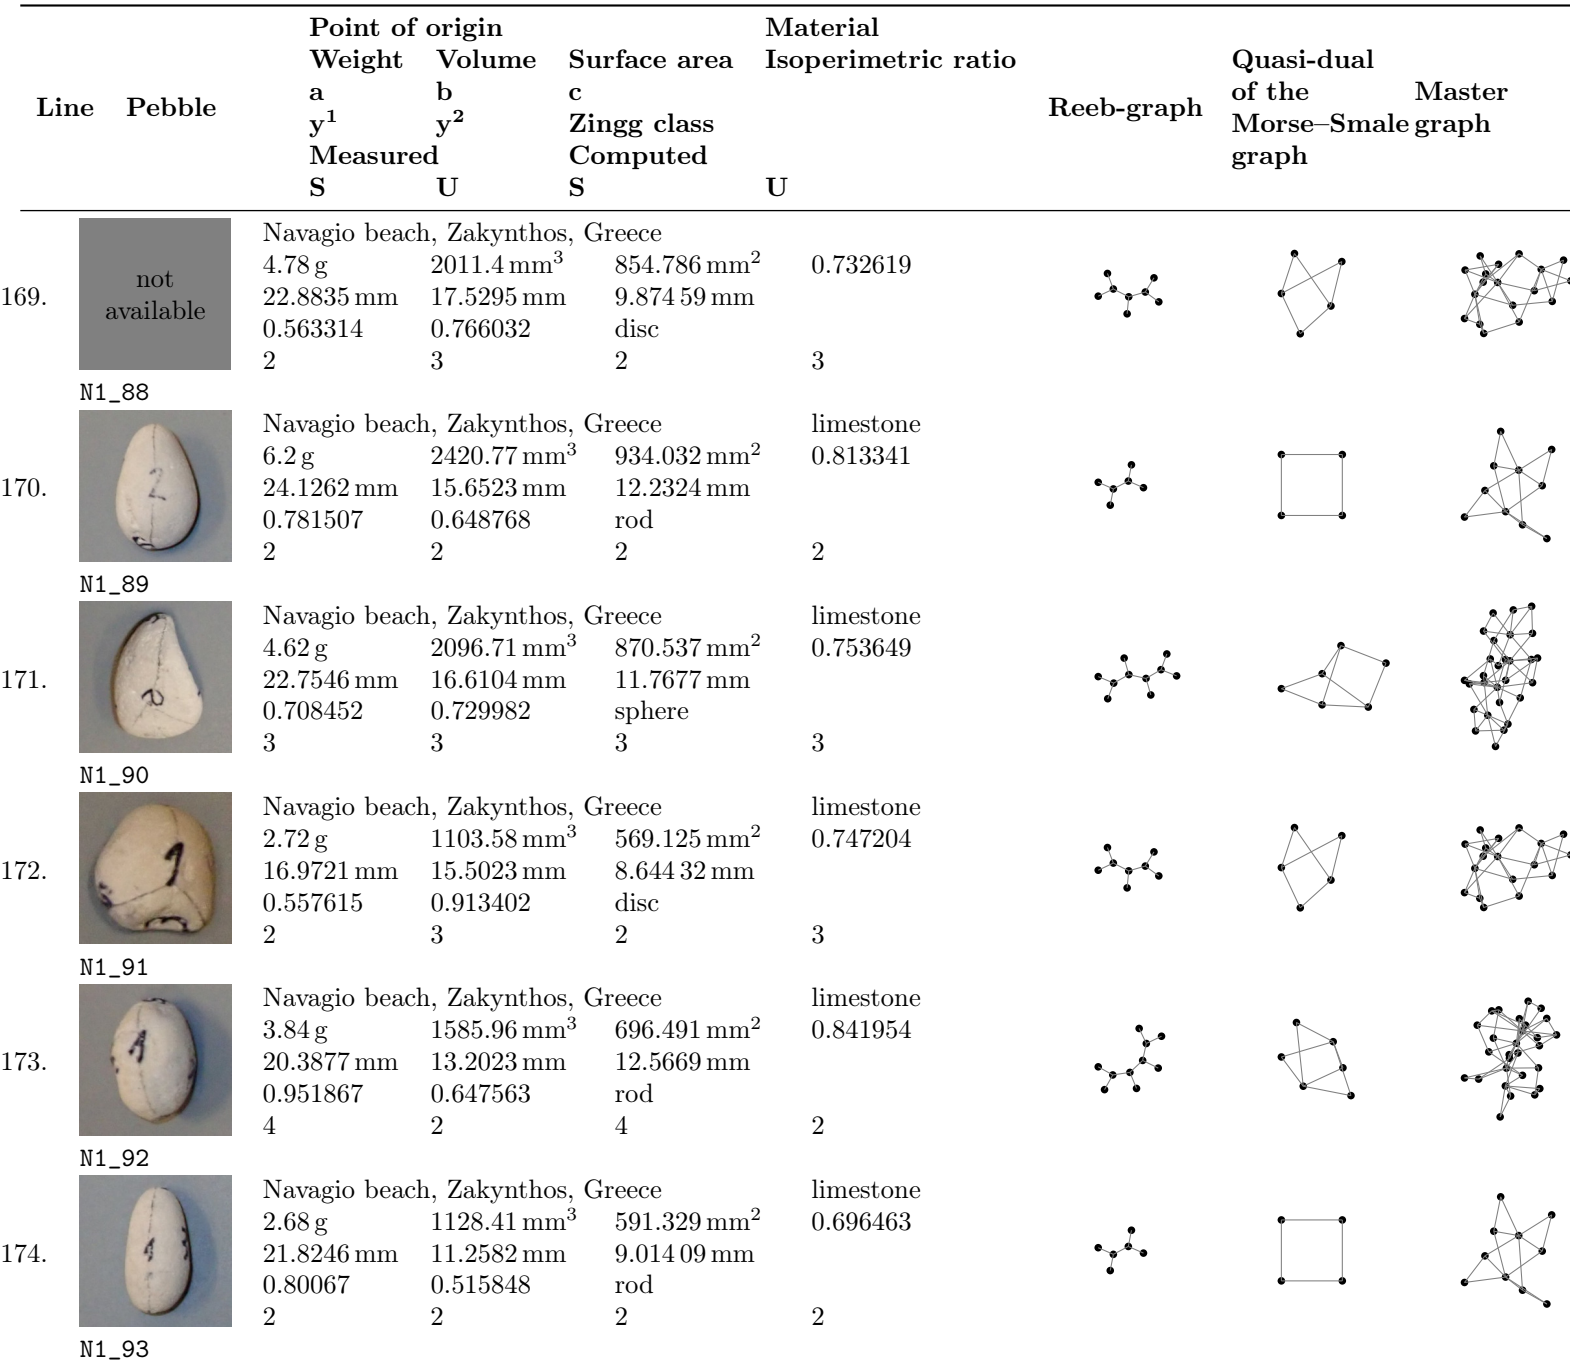 |
|      |                                                                                     | 3.84 g                           | 1585.96 mm <sup>3</sup> | 696.491 mm <sup>2</sup>      |           |                     |                                                                                       |                                                                                       |                                                                                       |
|      |                                                                                     | 20.3877 mm                       | 13.2023 mm              | 12.5669 mm                   |           |                     |                                                                                       |                                                                                       |                                                                                       |
|      |                                                                                     | 0.951867                         | 0.647563                | rod                          |           |                     |                                                                                       |                                                                                       |                                                                                       |
|      |                                                                                     | 4                                | 2                       | 4                            |           |                     |                                                                                       |                                                                                       |                                                                                       |
|      | N1_92                                                                               |                                  |                         |                              |           |                     |                                                                                       |                                                                                       |                                                                                       |
| 174. | 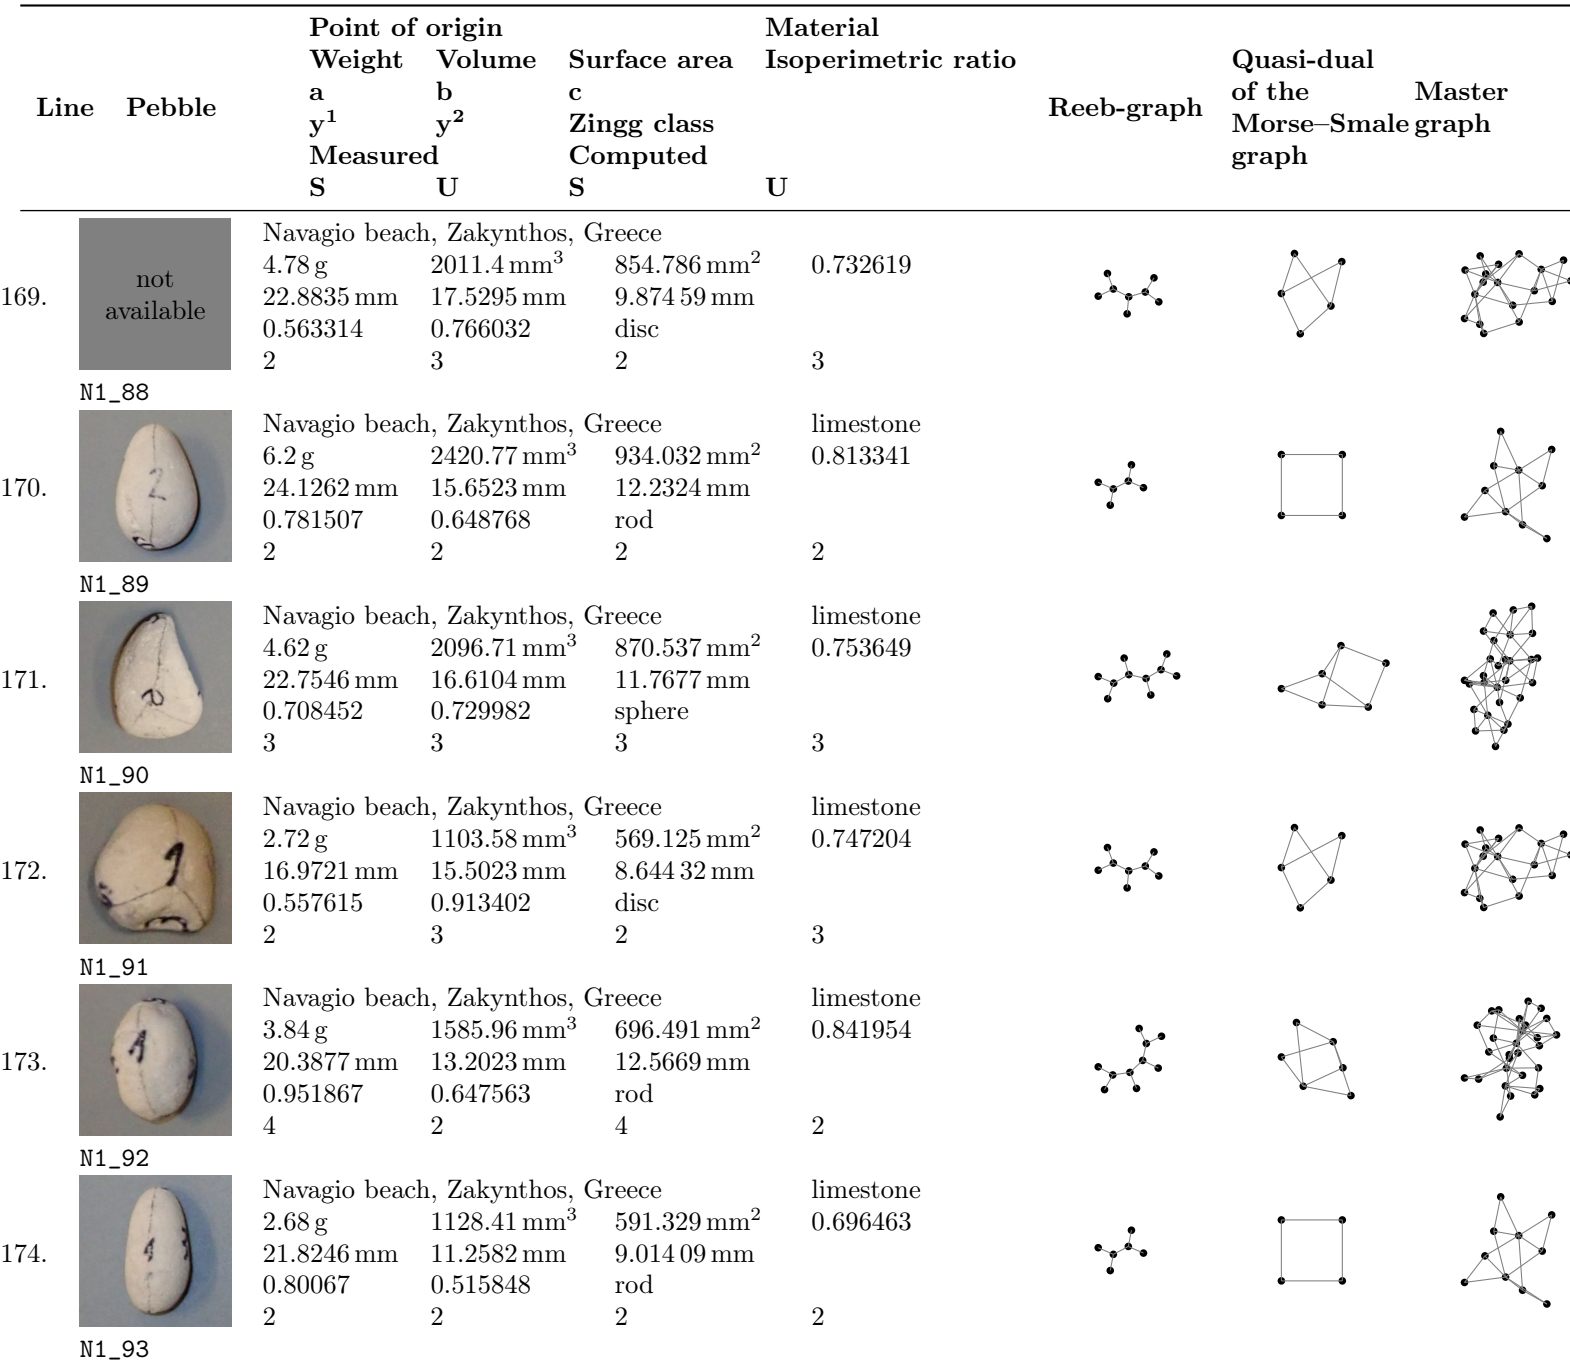 | Navagio beach, Zakynthos, Greece |                         |                              | limestone | 0.696463            | 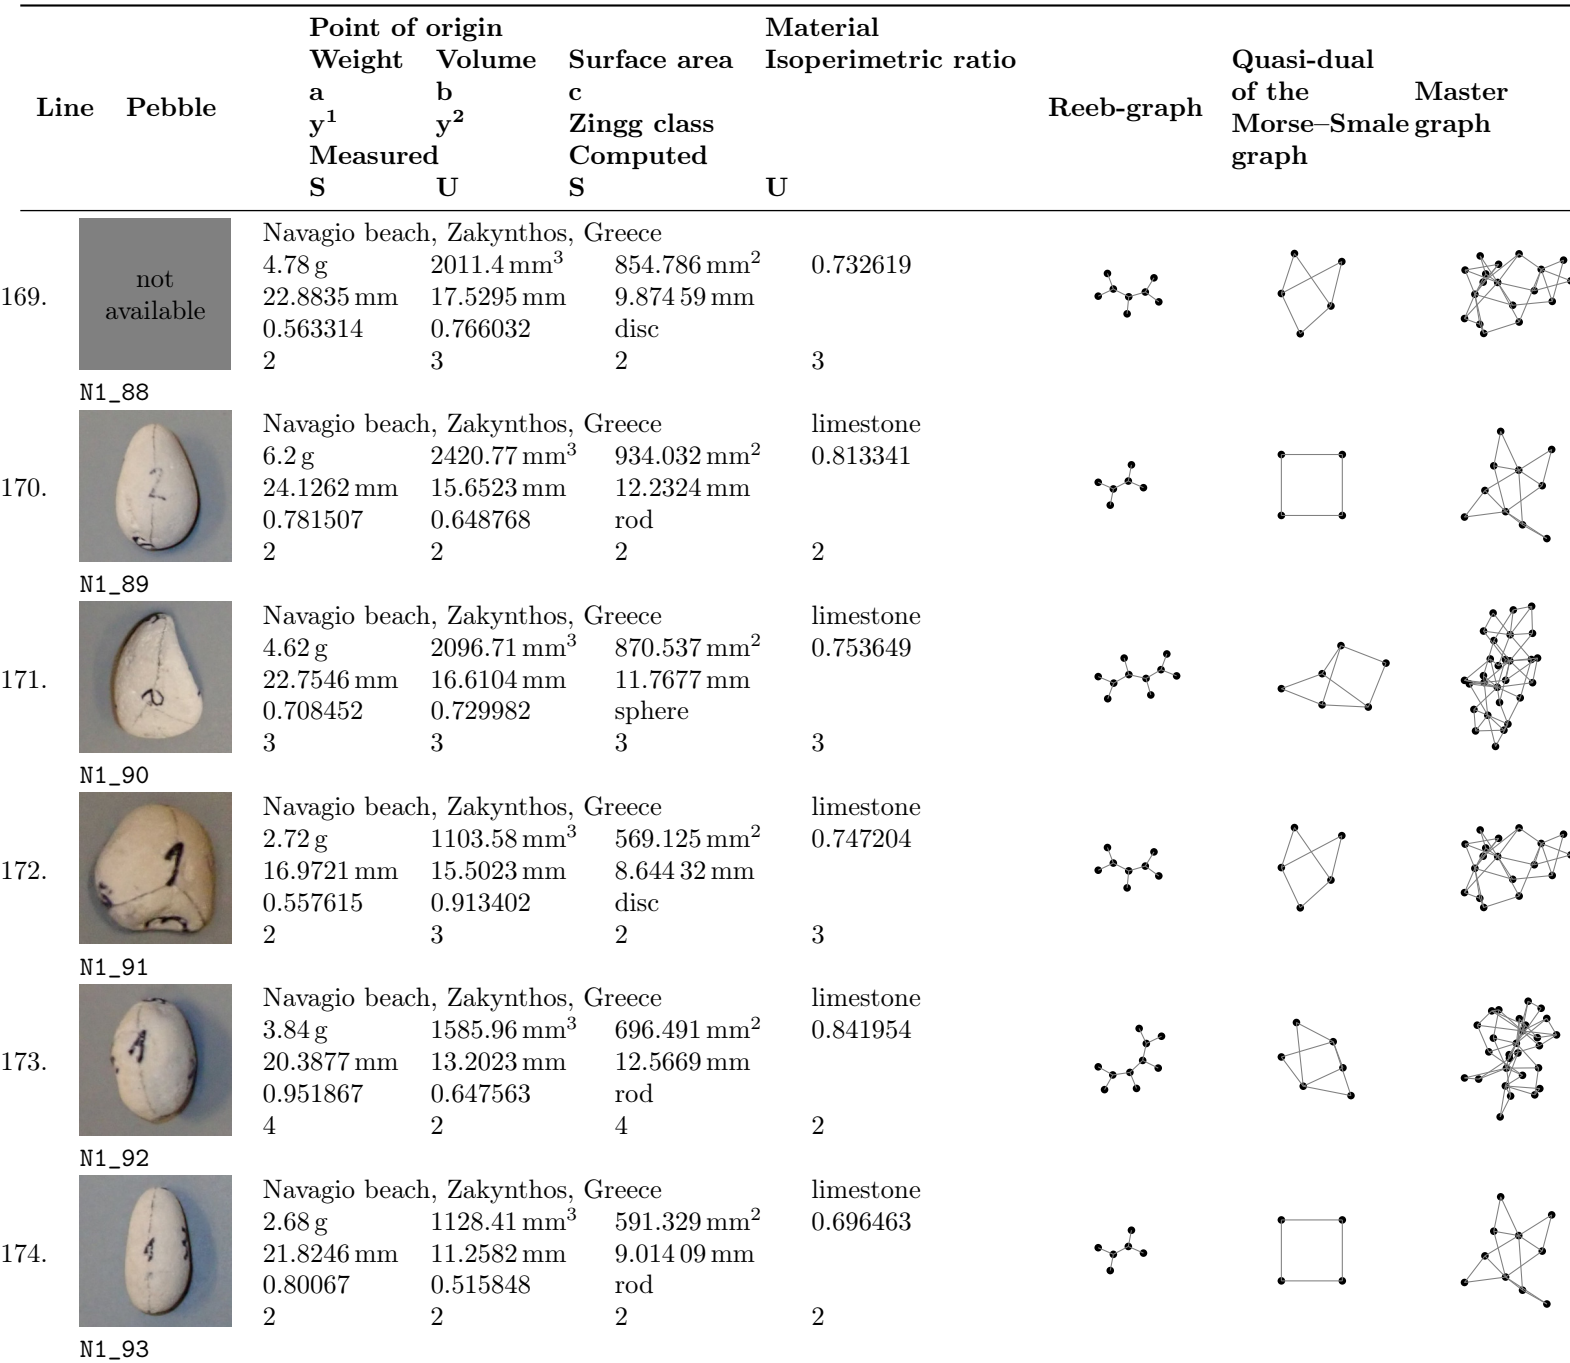 | 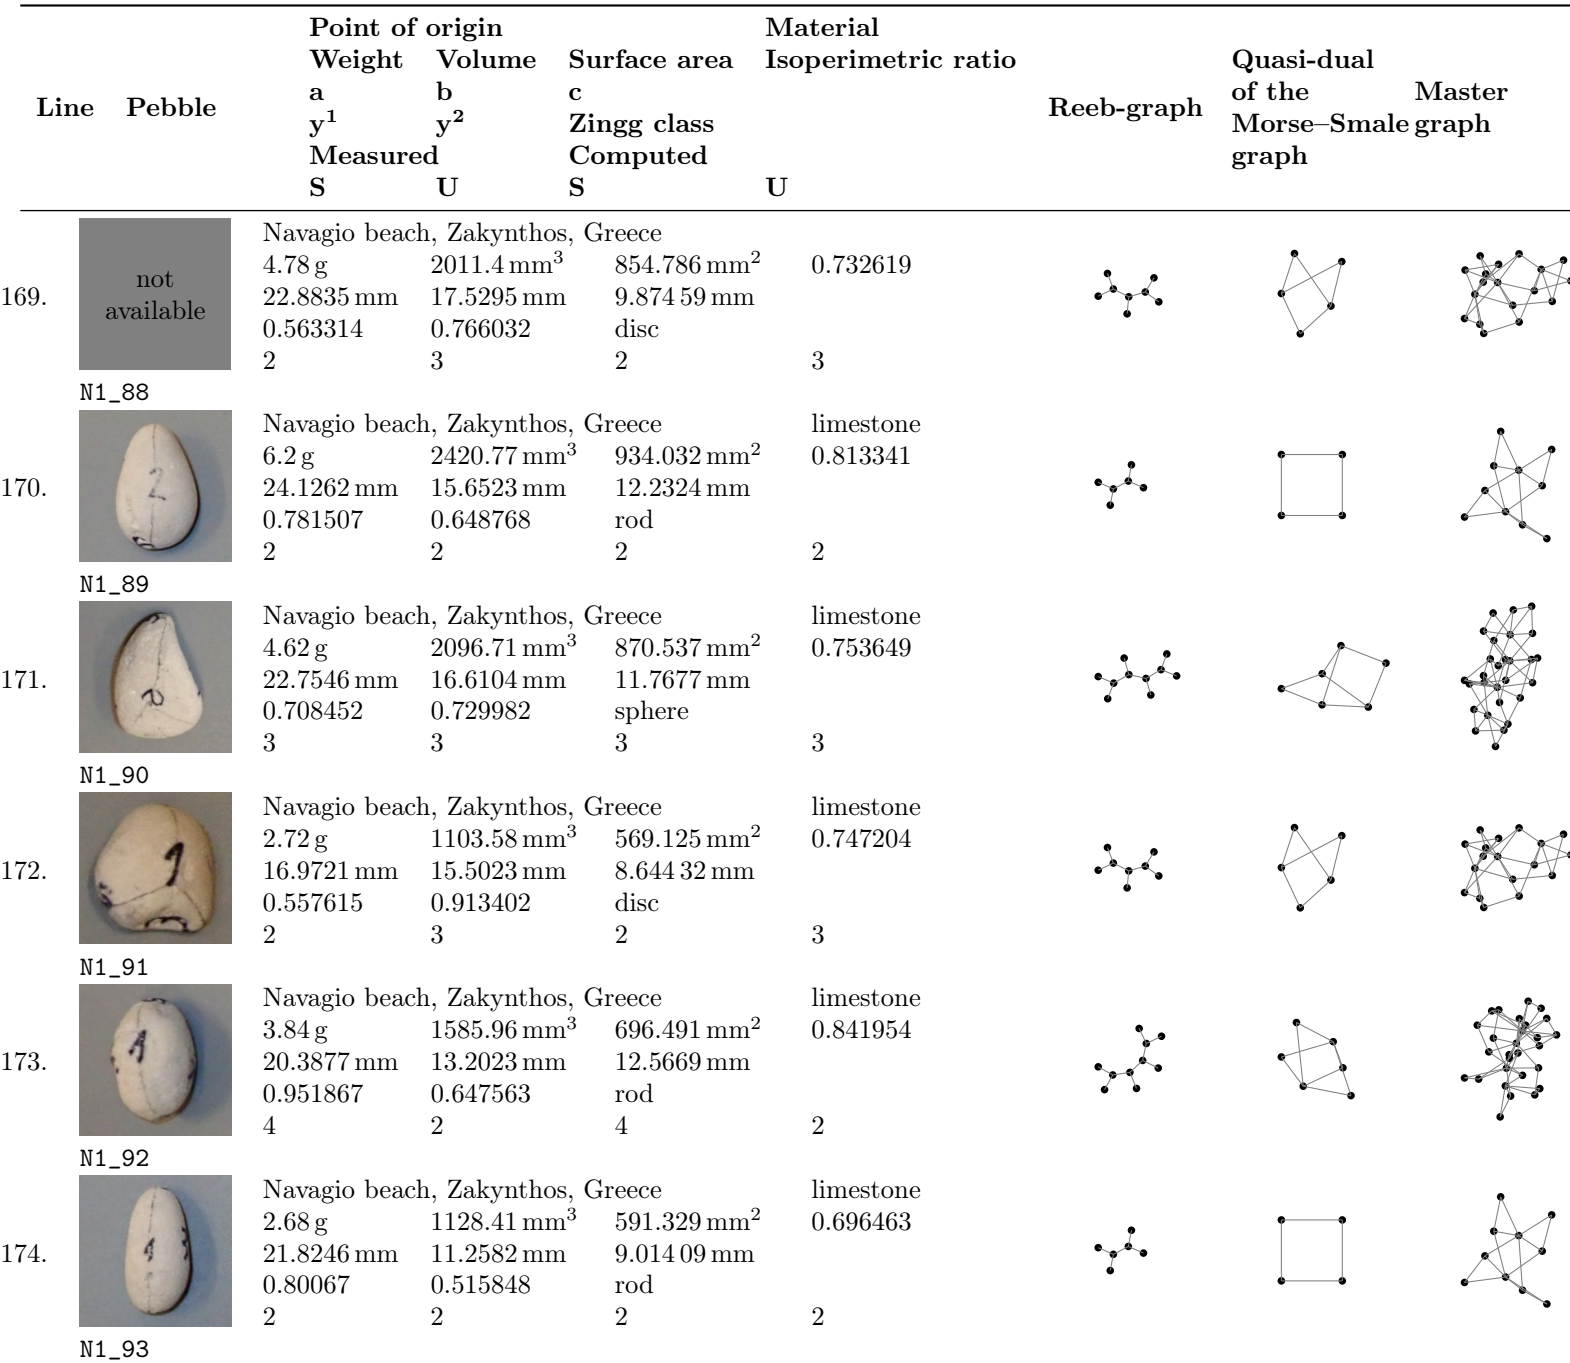 | 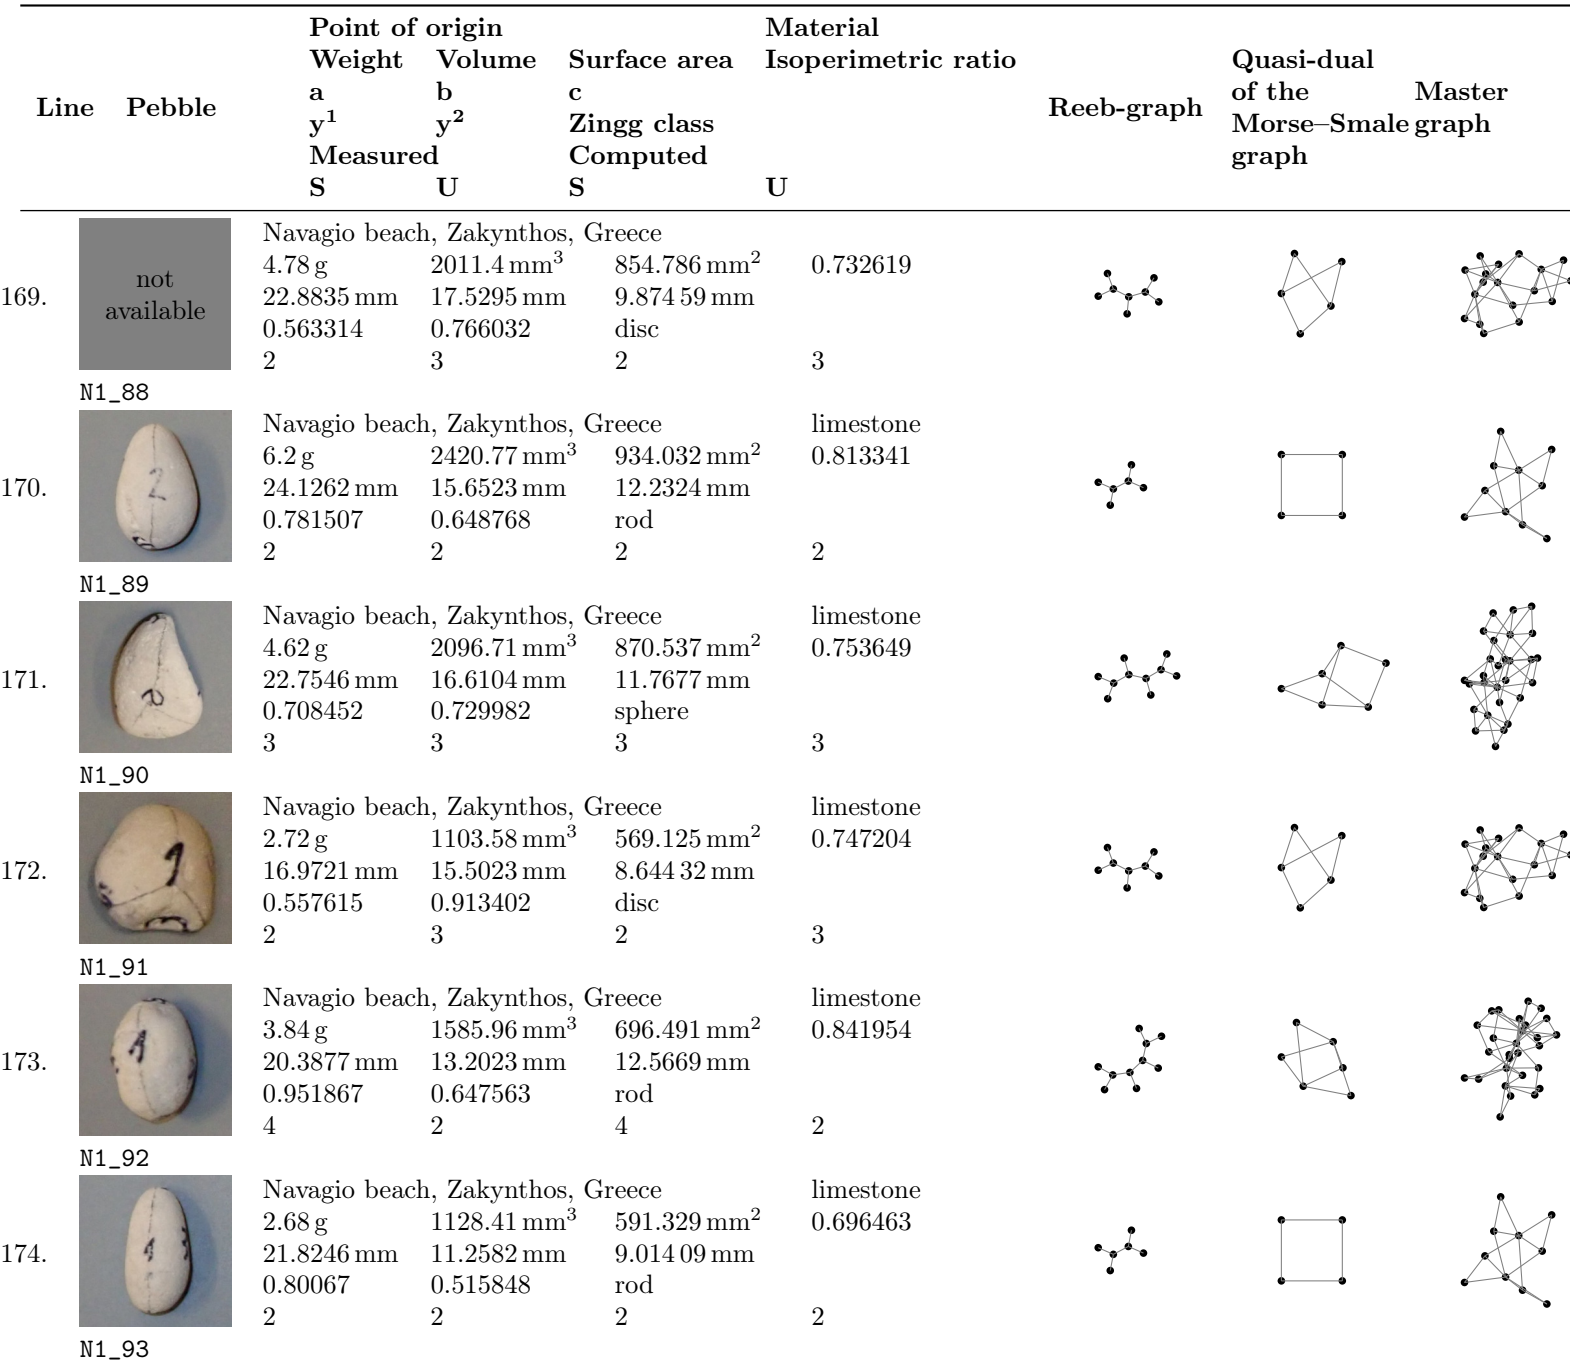 |
|      |                                                                                     | 2.68 g                           | 1128.41 mm <sup>3</sup> | 591.329 mm <sup>2</sup>      |           |                     |                                                                                       |                                                                                       |                                                                                       |
|      |                                                                                     | 21.8246 mm                       | 11.2582 mm              | 9.014 09 mm                  |           |                     |                                                                                       |                                                                                       |                                                                                       |
|      |                                                                                     | 0.80067                          | 0.515848                | rod                          |           |                     |                                                                                       |                                                                                       |                                                                                       |
|      |                                                                                     | 2                                | 2                       | 2                            |           |                     |                                                                                       |                                                                                       |                                                                                       |
|      | N1_93                                                                               |                                  |                         |                              |           |                     |                                                                                       |                                                                                       |                                                                                       |

| Line | Pebble                                                                              | Point of origin                      |                          | Surface area<br>c<br>Zingg class<br>Computed<br>S | Material<br>Isoperimetric ratio<br>U | Reeb-graph                                                                            | Quasi-dual<br>of the<br>Morse–Smale<br>graph                                          | Master<br>graph                                                                       |
|------|-------------------------------------------------------------------------------------|--------------------------------------|--------------------------|---------------------------------------------------|--------------------------------------|---------------------------------------------------------------------------------------|---------------------------------------------------------------------------------------|---------------------------------------------------------------------------------------|
|      |                                                                                     | Weight                               | Volume                   |                                                   |                                      |                                                                                       |                                                                                       |                                                                                       |
|      |                                                                                     | a<br>y <sup>1</sup><br>Measured<br>S | b<br>y <sup>2</sup><br>U |                                                   |                                      |                                                                                       |                                                                                       |                                                                                       |
|      |                                                                                     |                                      |                          |                                                   |                                      |                                                                                       |                                                                                       |                                                                                       |
| 175. | 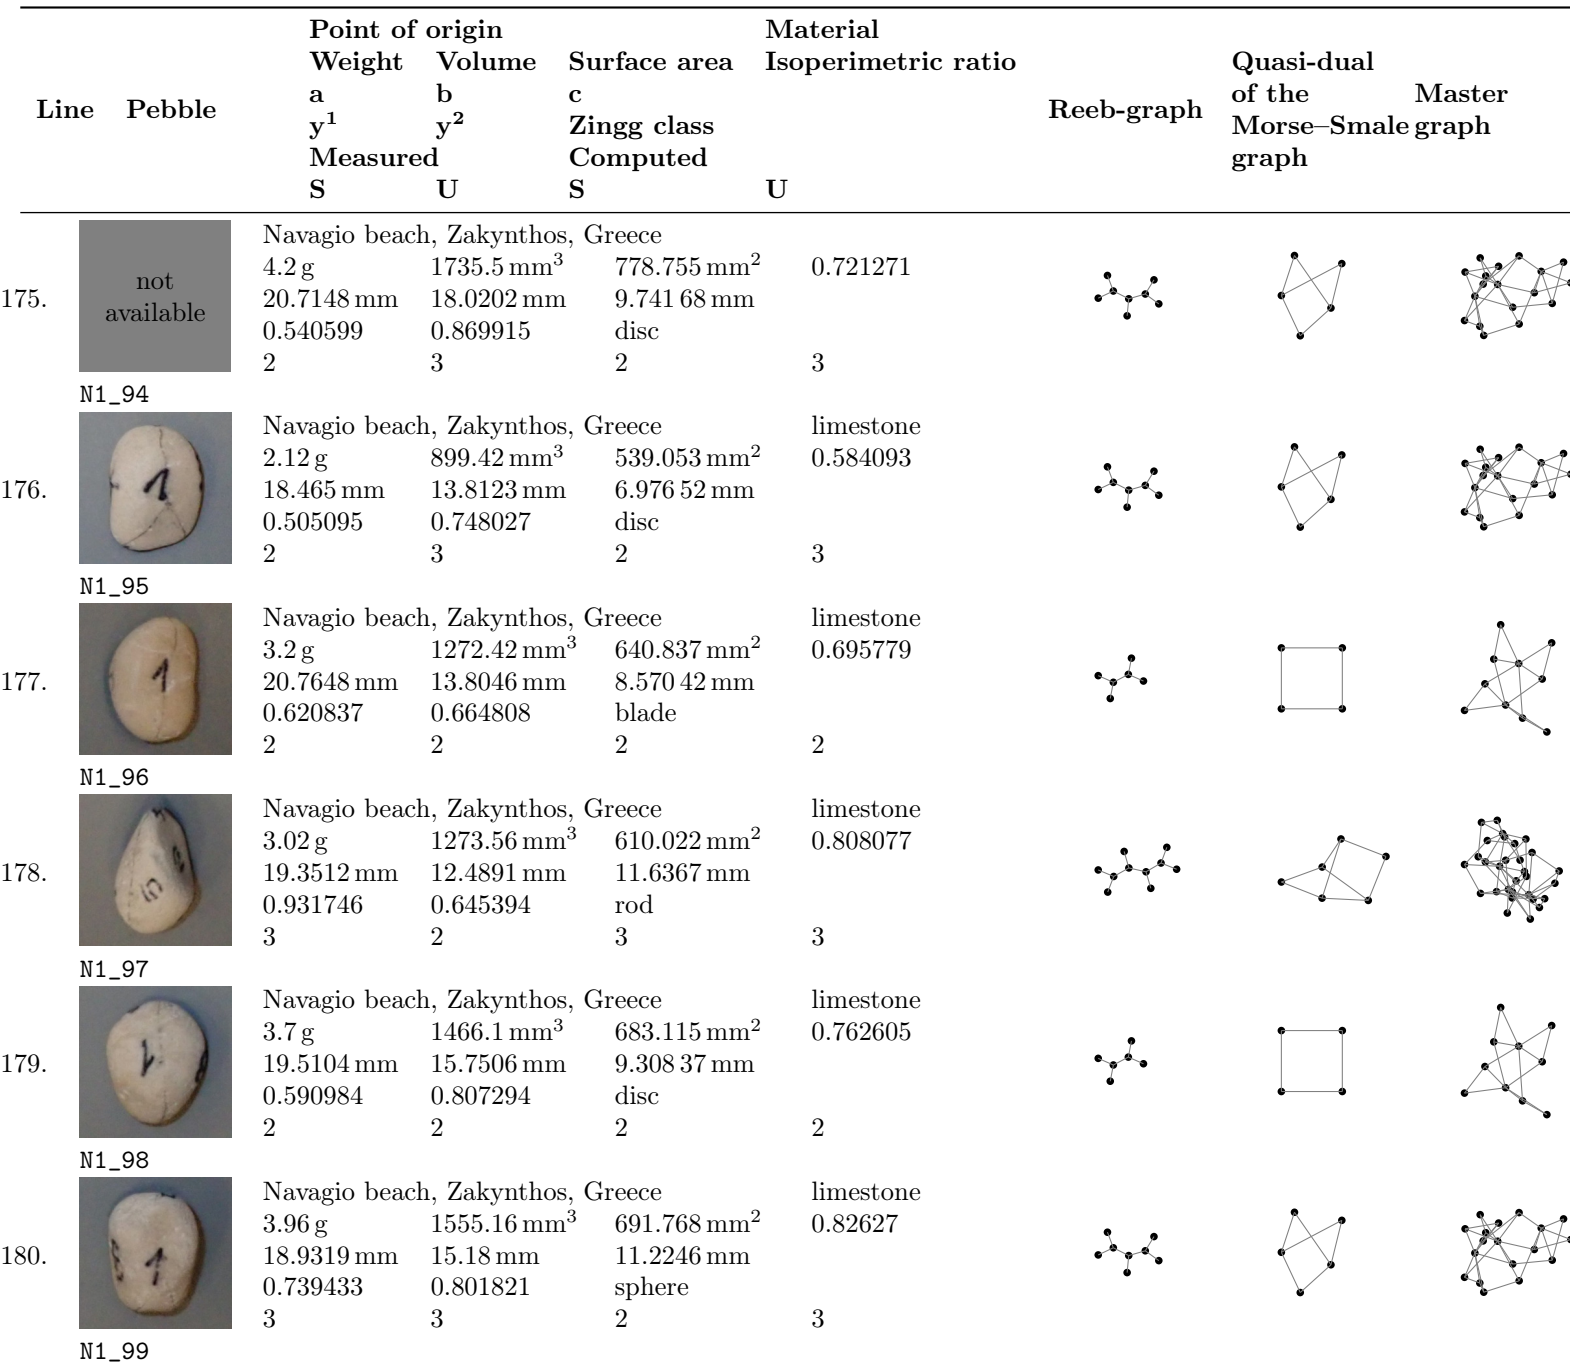   | Navagio beach, Zakynthos, Greece     |                          |                                                   | 0.721271                             | 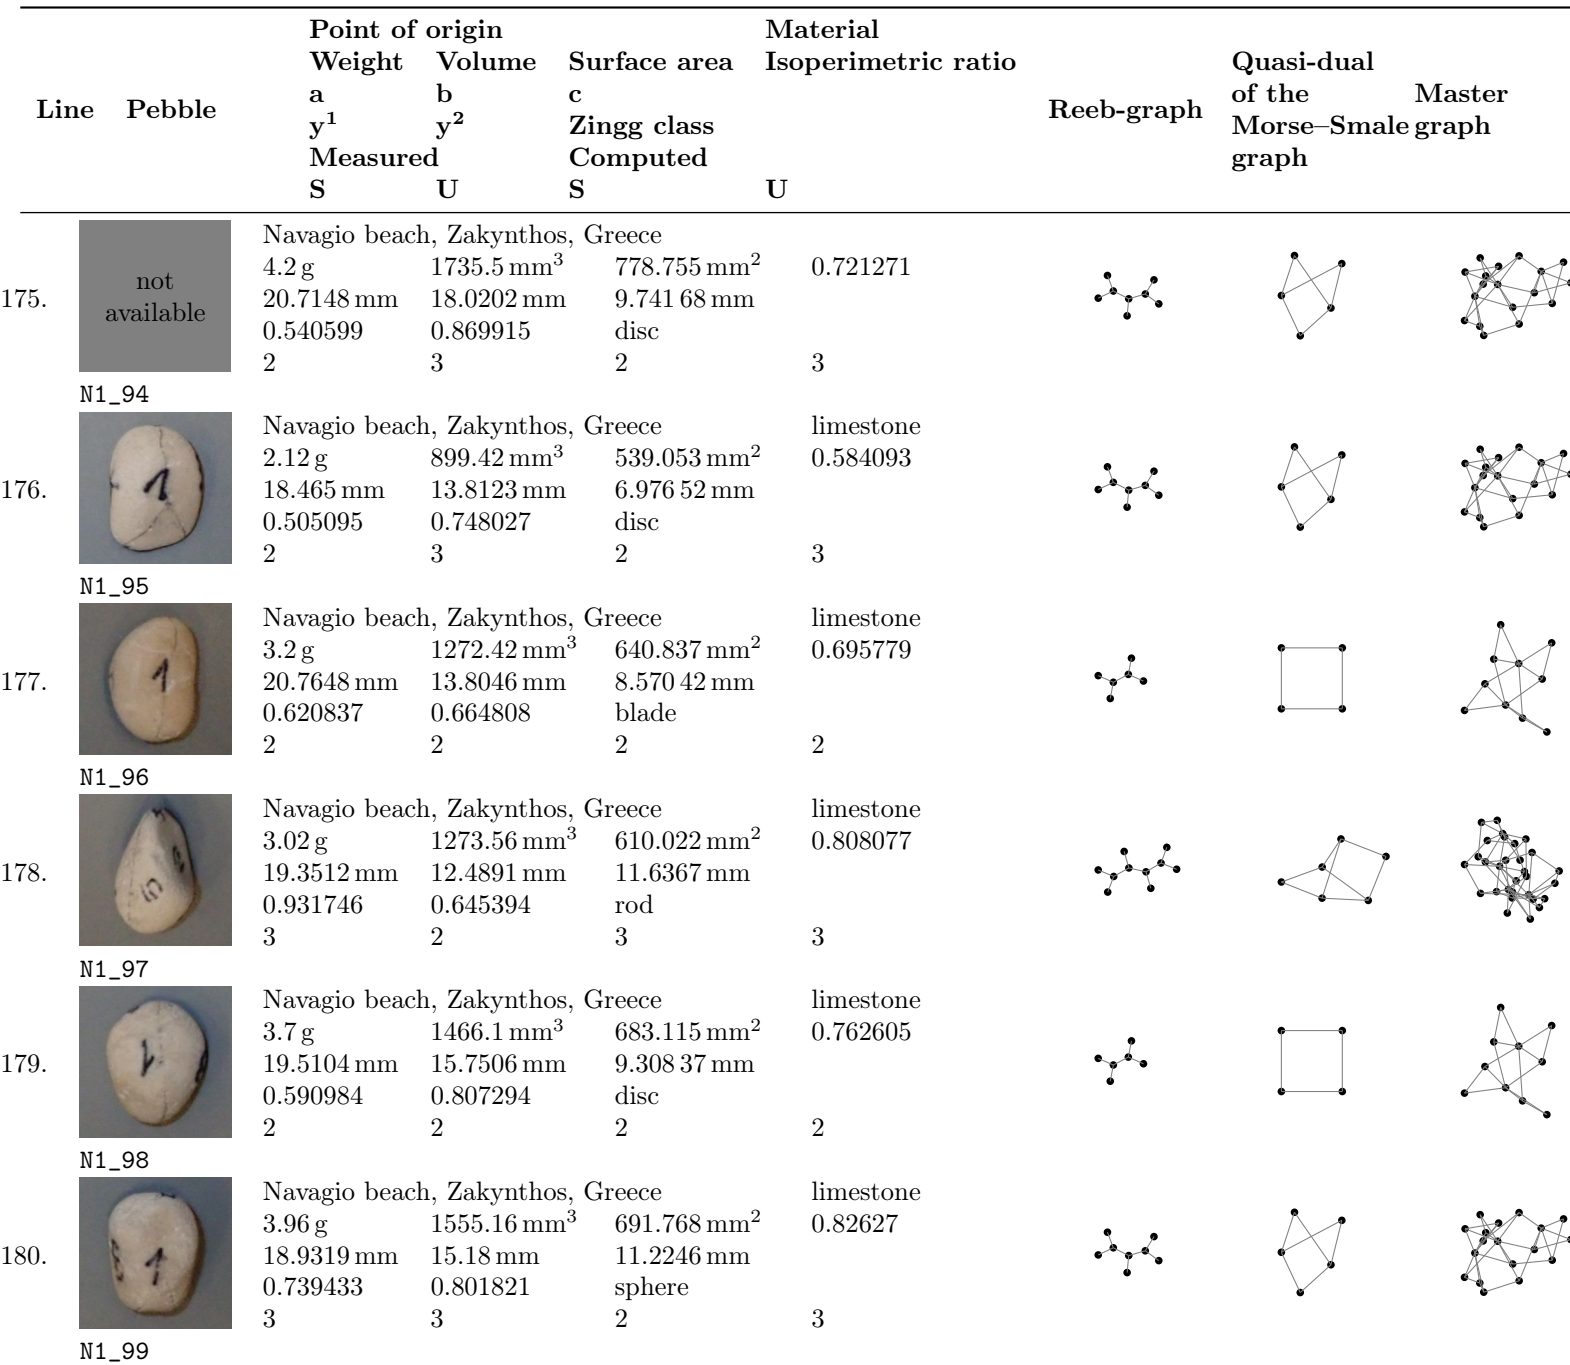   | 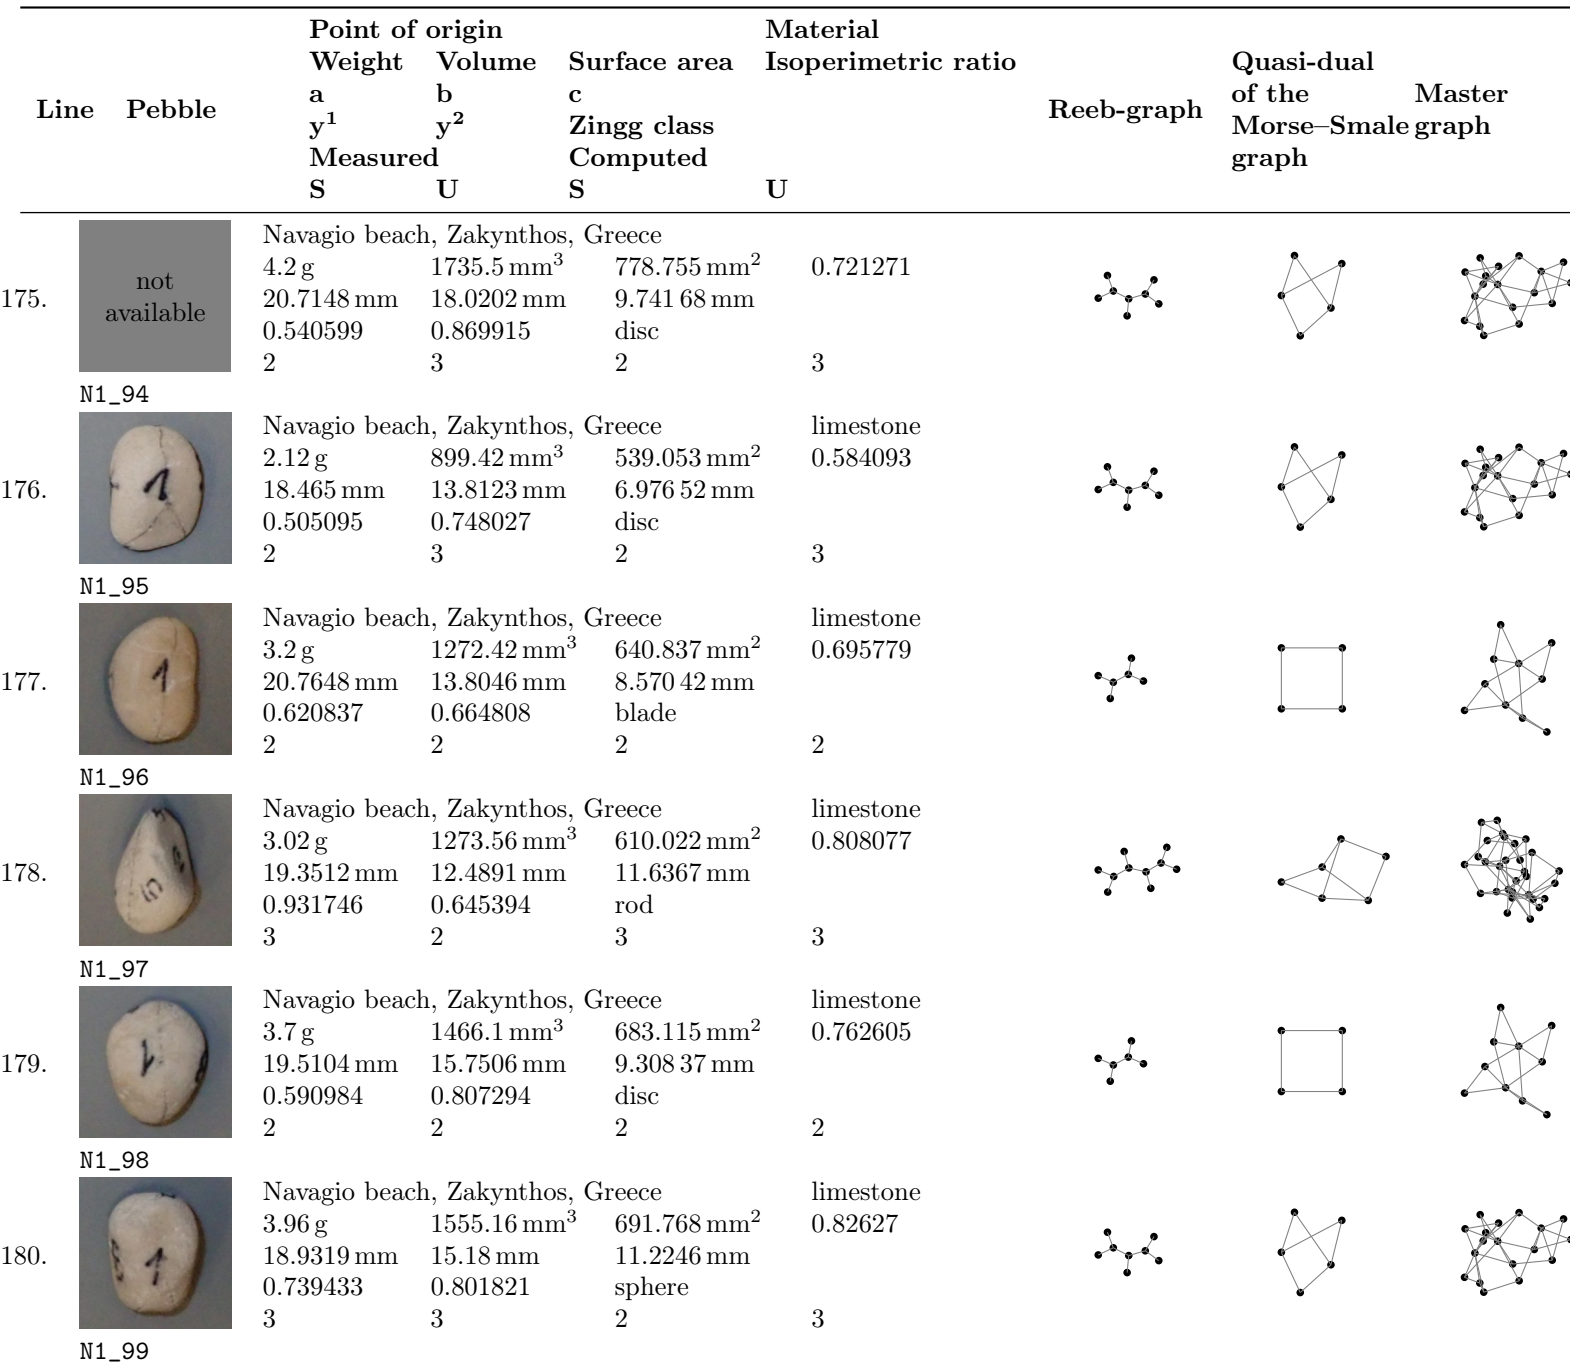   | 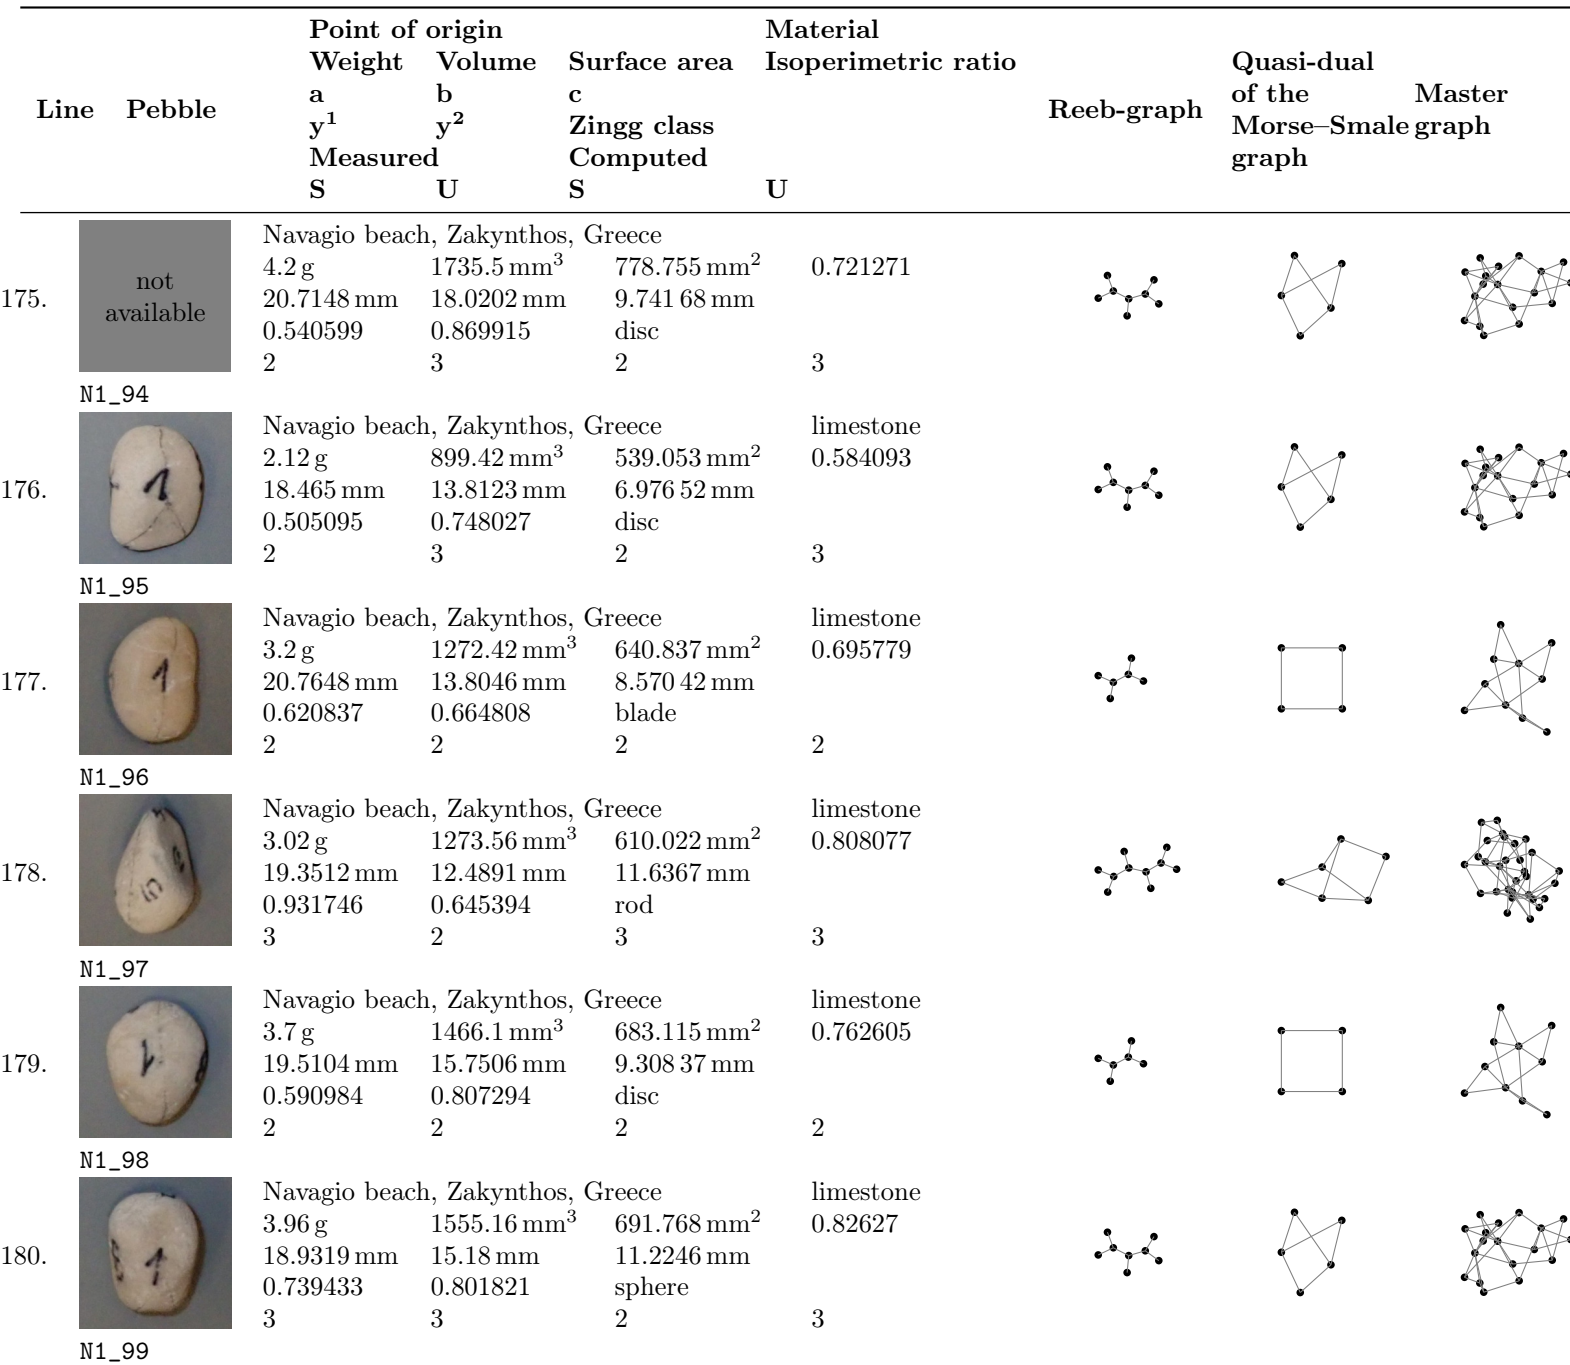   |
|      |                                                                                     | 4.2 g                                | 1735.5 mm <sup>3</sup>   | 778.755 mm <sup>2</sup>                           |                                      |                                                                                       |                                                                                       |                                                                                       |
|      |                                                                                     | 20.7148 mm                           | 18.0202 mm               | 9.741 68 mm                                       |                                      |                                                                                       |                                                                                       |                                                                                       |
|      |                                                                                     | 0.540599                             | 0.869915                 | disc                                              |                                      |                                                                                       |                                                                                       |                                                                                       |
|      |                                                                                     | 2                                    | 3                        | 2                                                 |                                      |                                                                                       |                                                                                       |                                                                                       |
|      | N1_94                                                                               |                                      |                          |                                                   |                                      |                                                                                       |                                                                                       |                                                                                       |
| 176. | 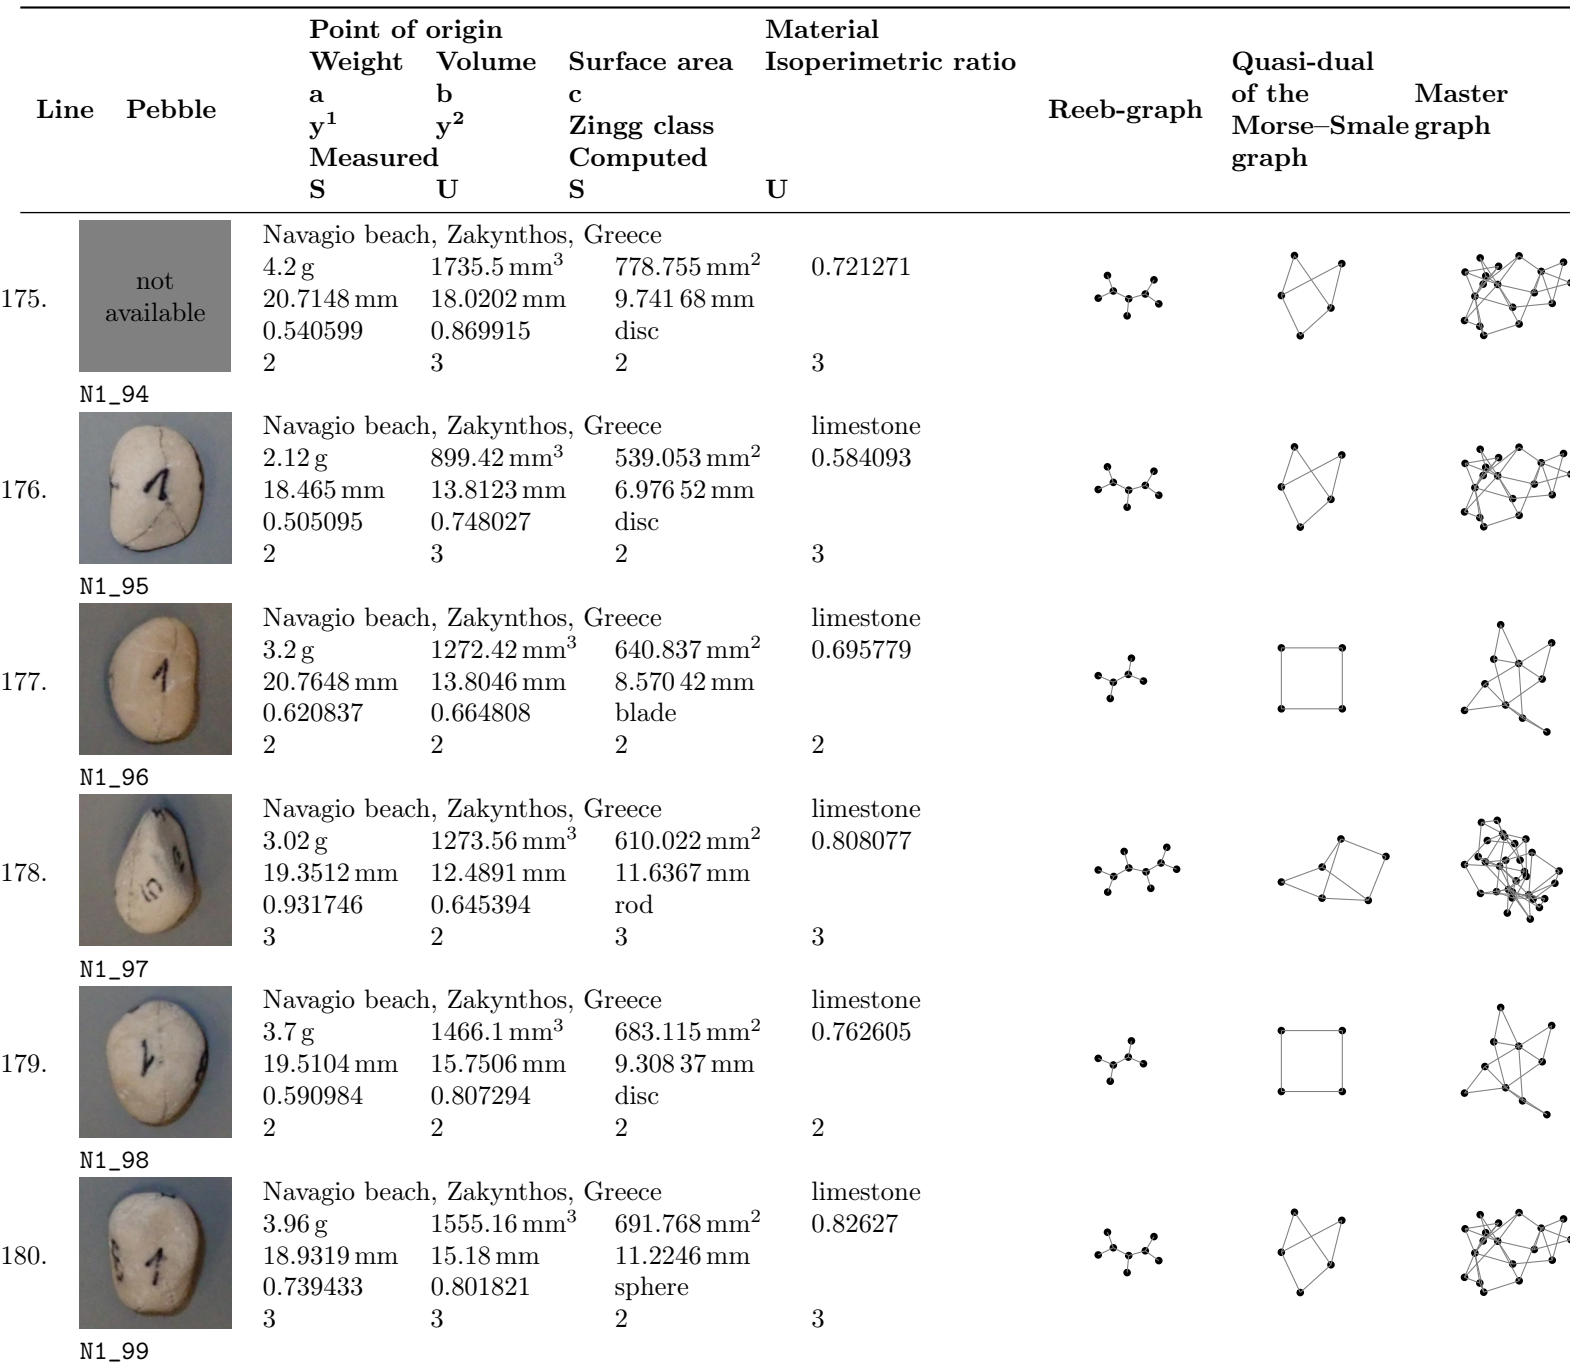   | Navagio beach, Zakynthos, Greece     |                          |                                                   | limestone<br>0.584093                | 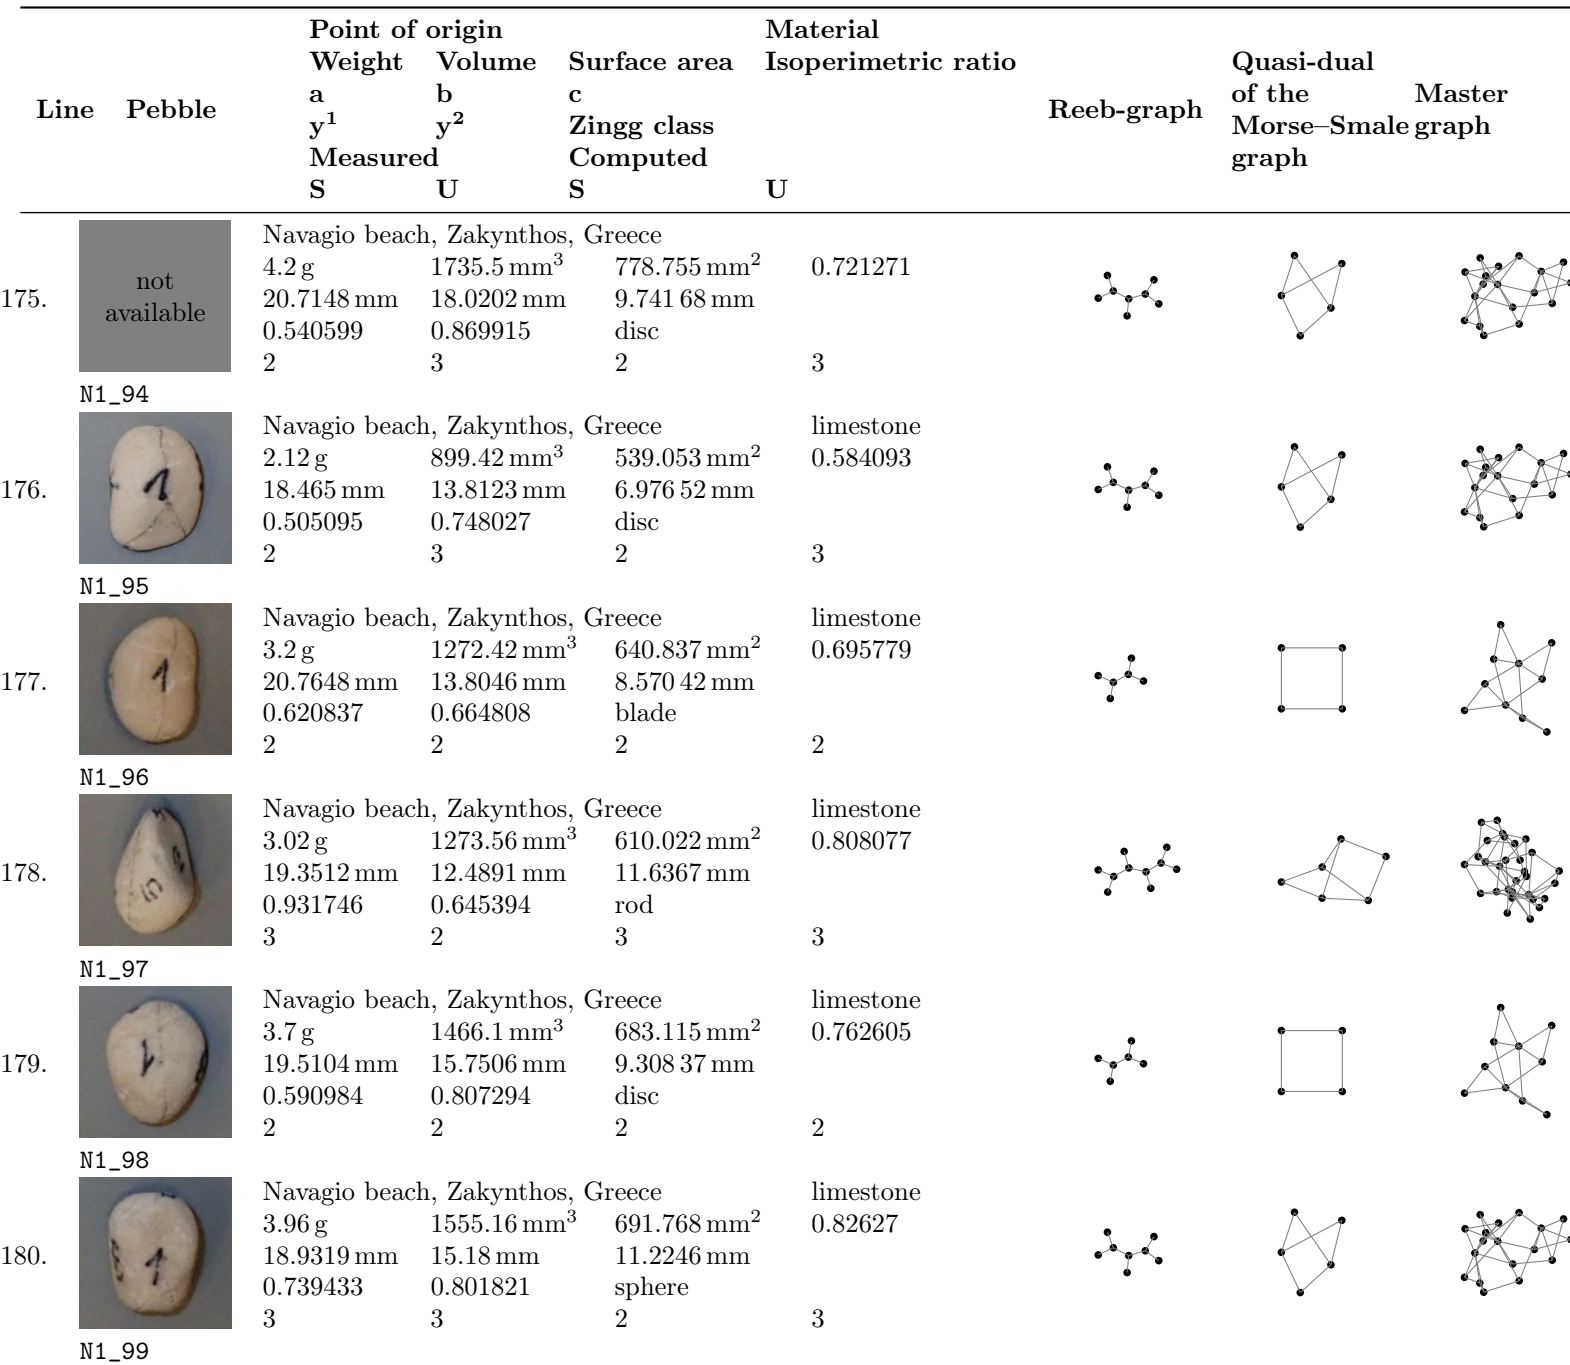   | 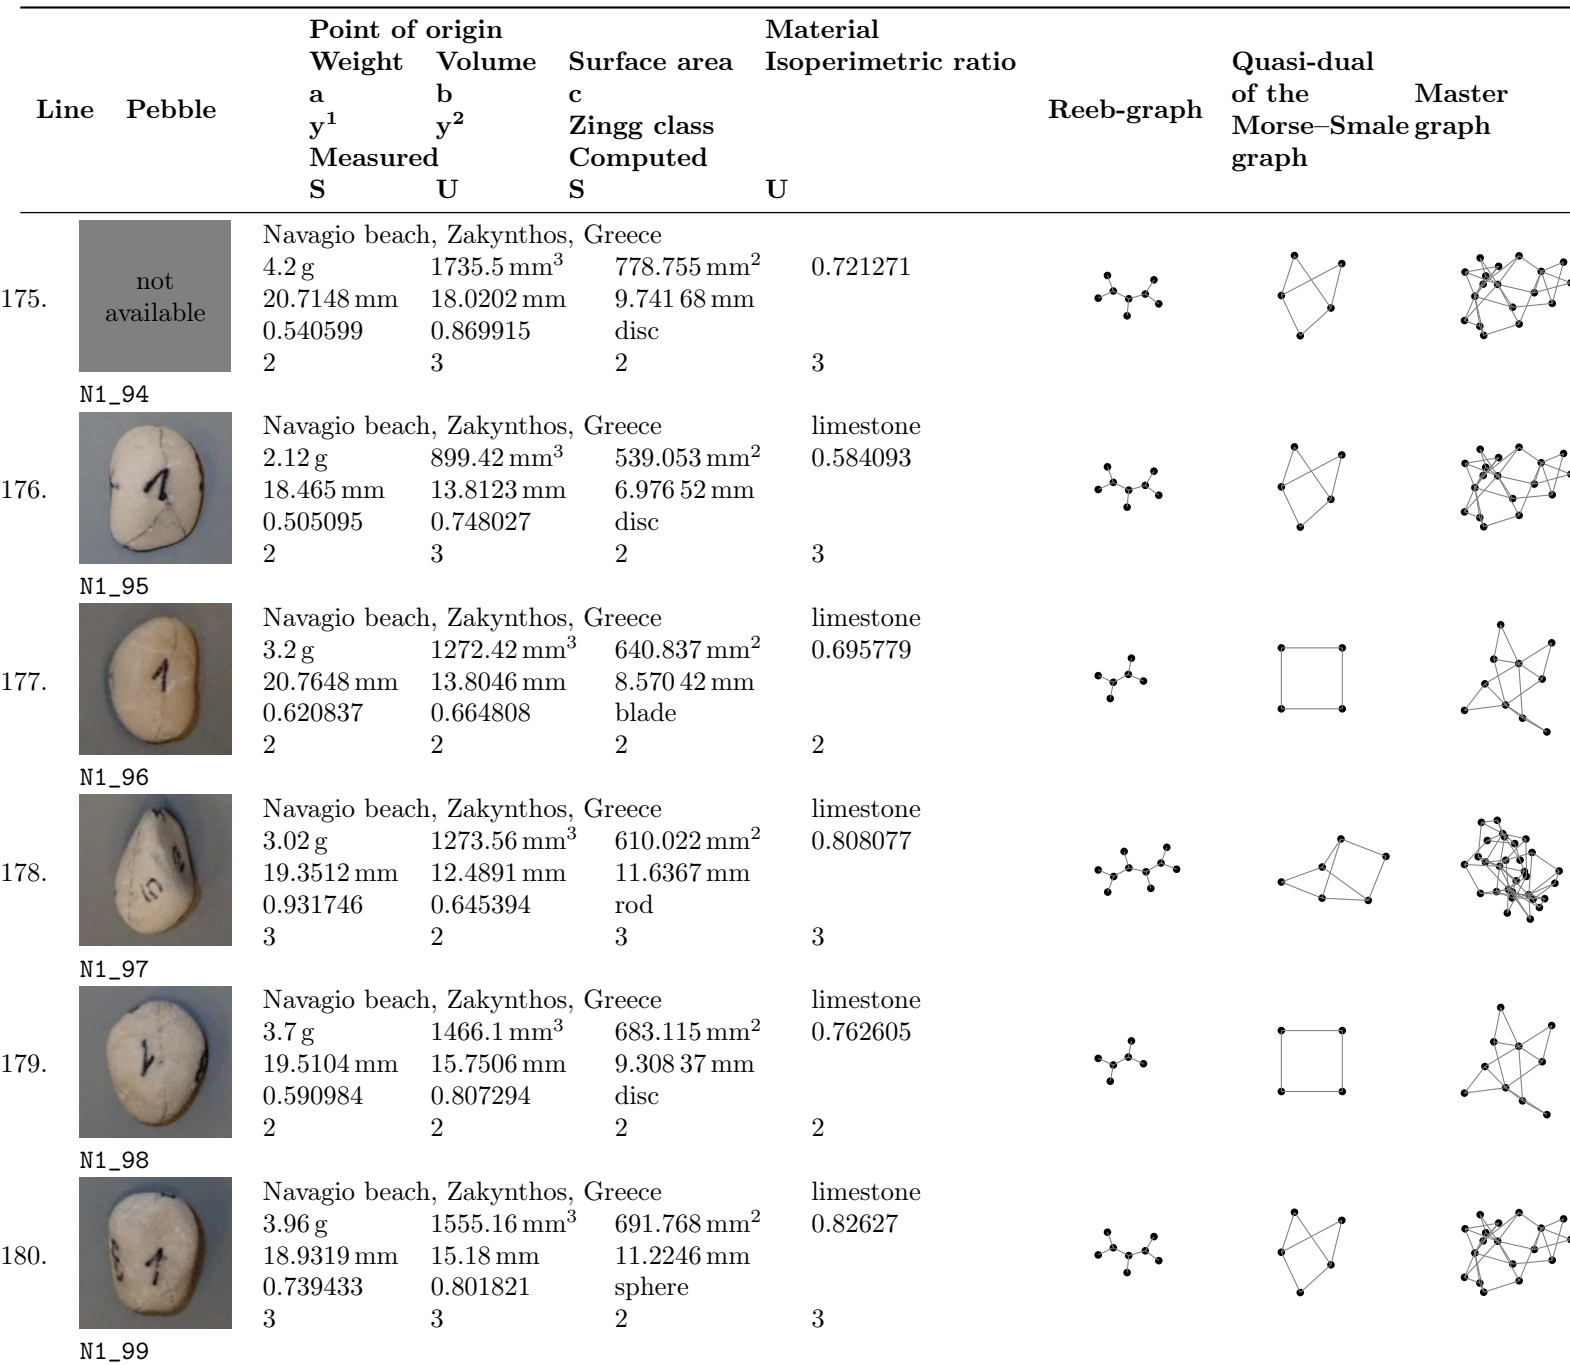   | 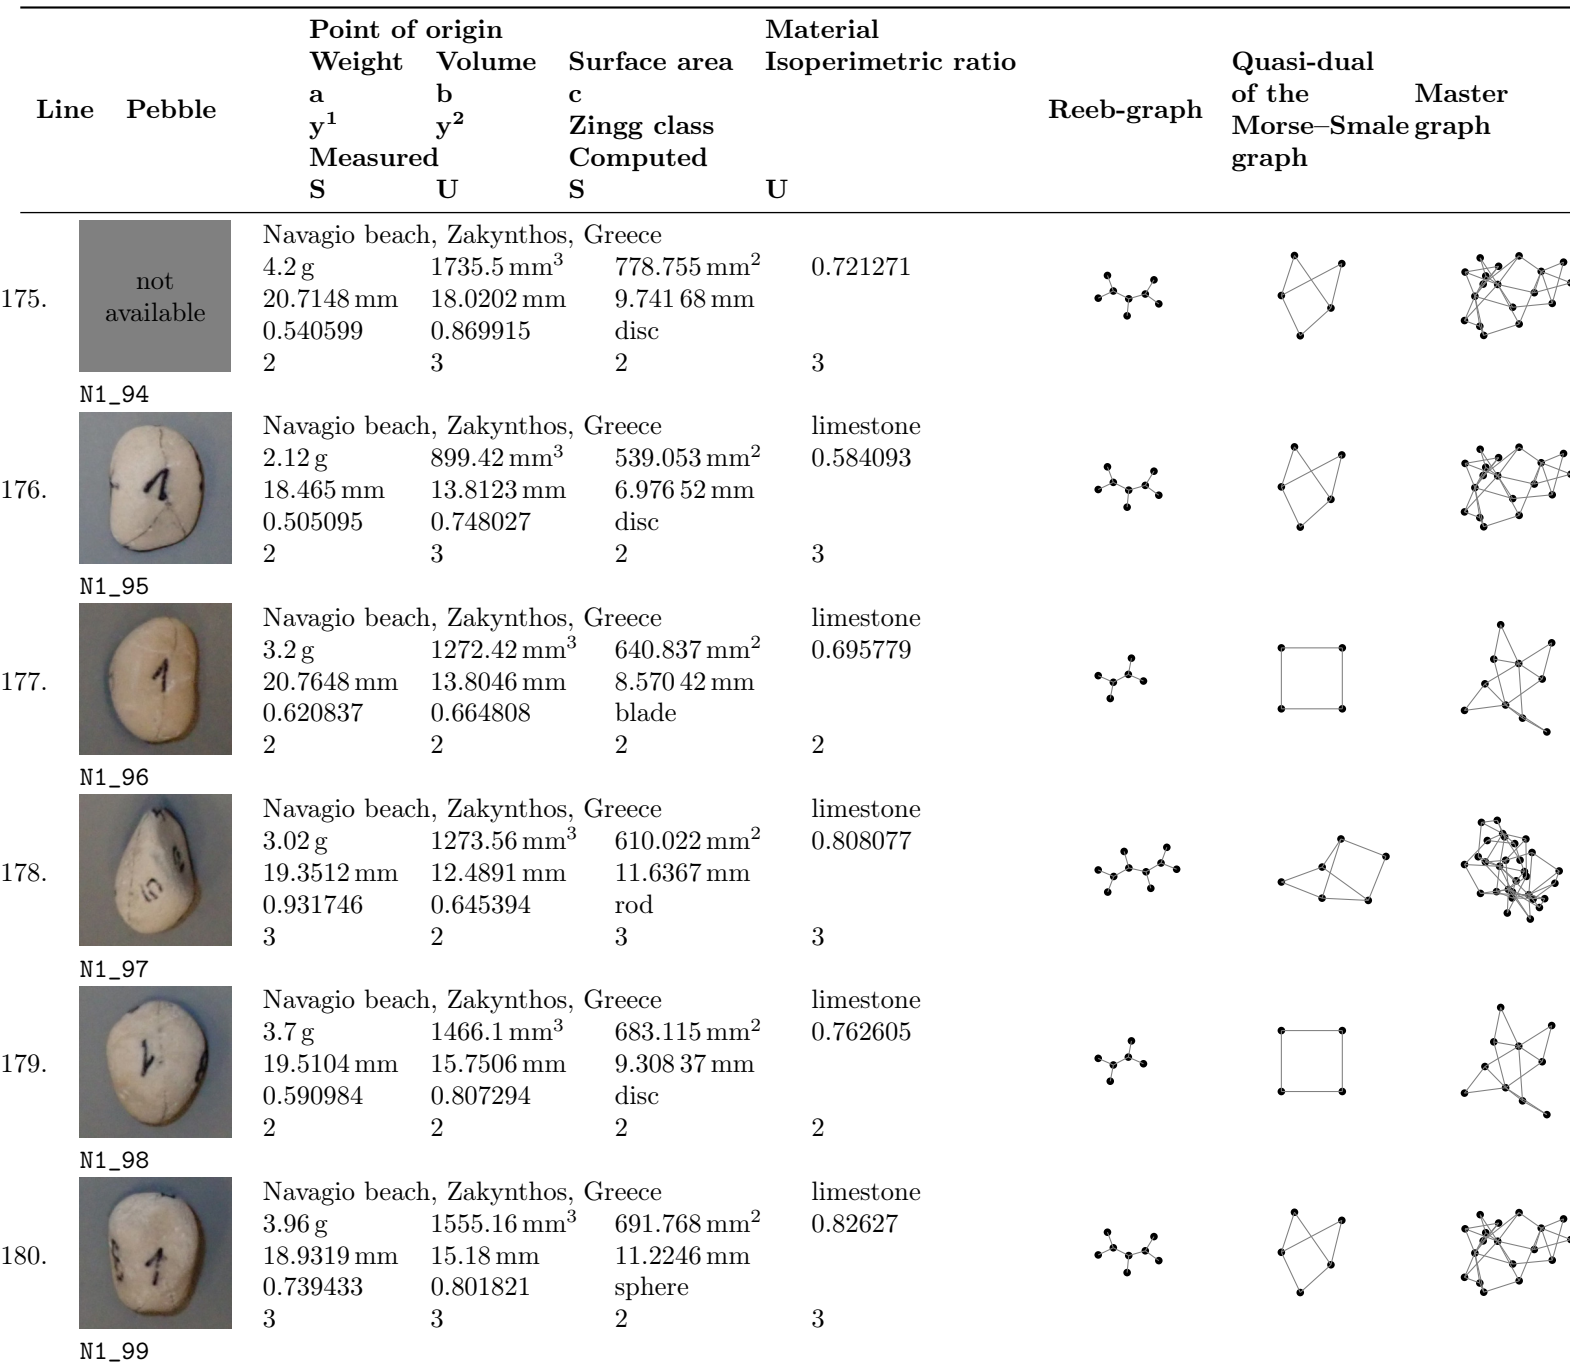   |
|      |                                                                                     | 2.12 g                               | 899.42 mm <sup>3</sup>   | 539.053 mm <sup>2</sup>                           |                                      |                                                                                       |                                                                                       |                                                                                       |
|      |                                                                                     | 18.465 mm                            | 13.8123 mm               | 6.976 52 mm                                       |                                      |                                                                                       |                                                                                       |                                                                                       |
|      |                                                                                     | 0.505095                             | 0.748027                 | disc                                              |                                      |                                                                                       |                                                                                       |                                                                                       |
|      |                                                                                     | 2                                    | 3                        | 2                                                 |                                      |                                                                                       |                                                                                       |                                                                                       |
|      | N1_95                                                                               |                                      |                          |                                                   |                                      |                                                                                       |                                                                                       |                                                                                       |
| 177. | 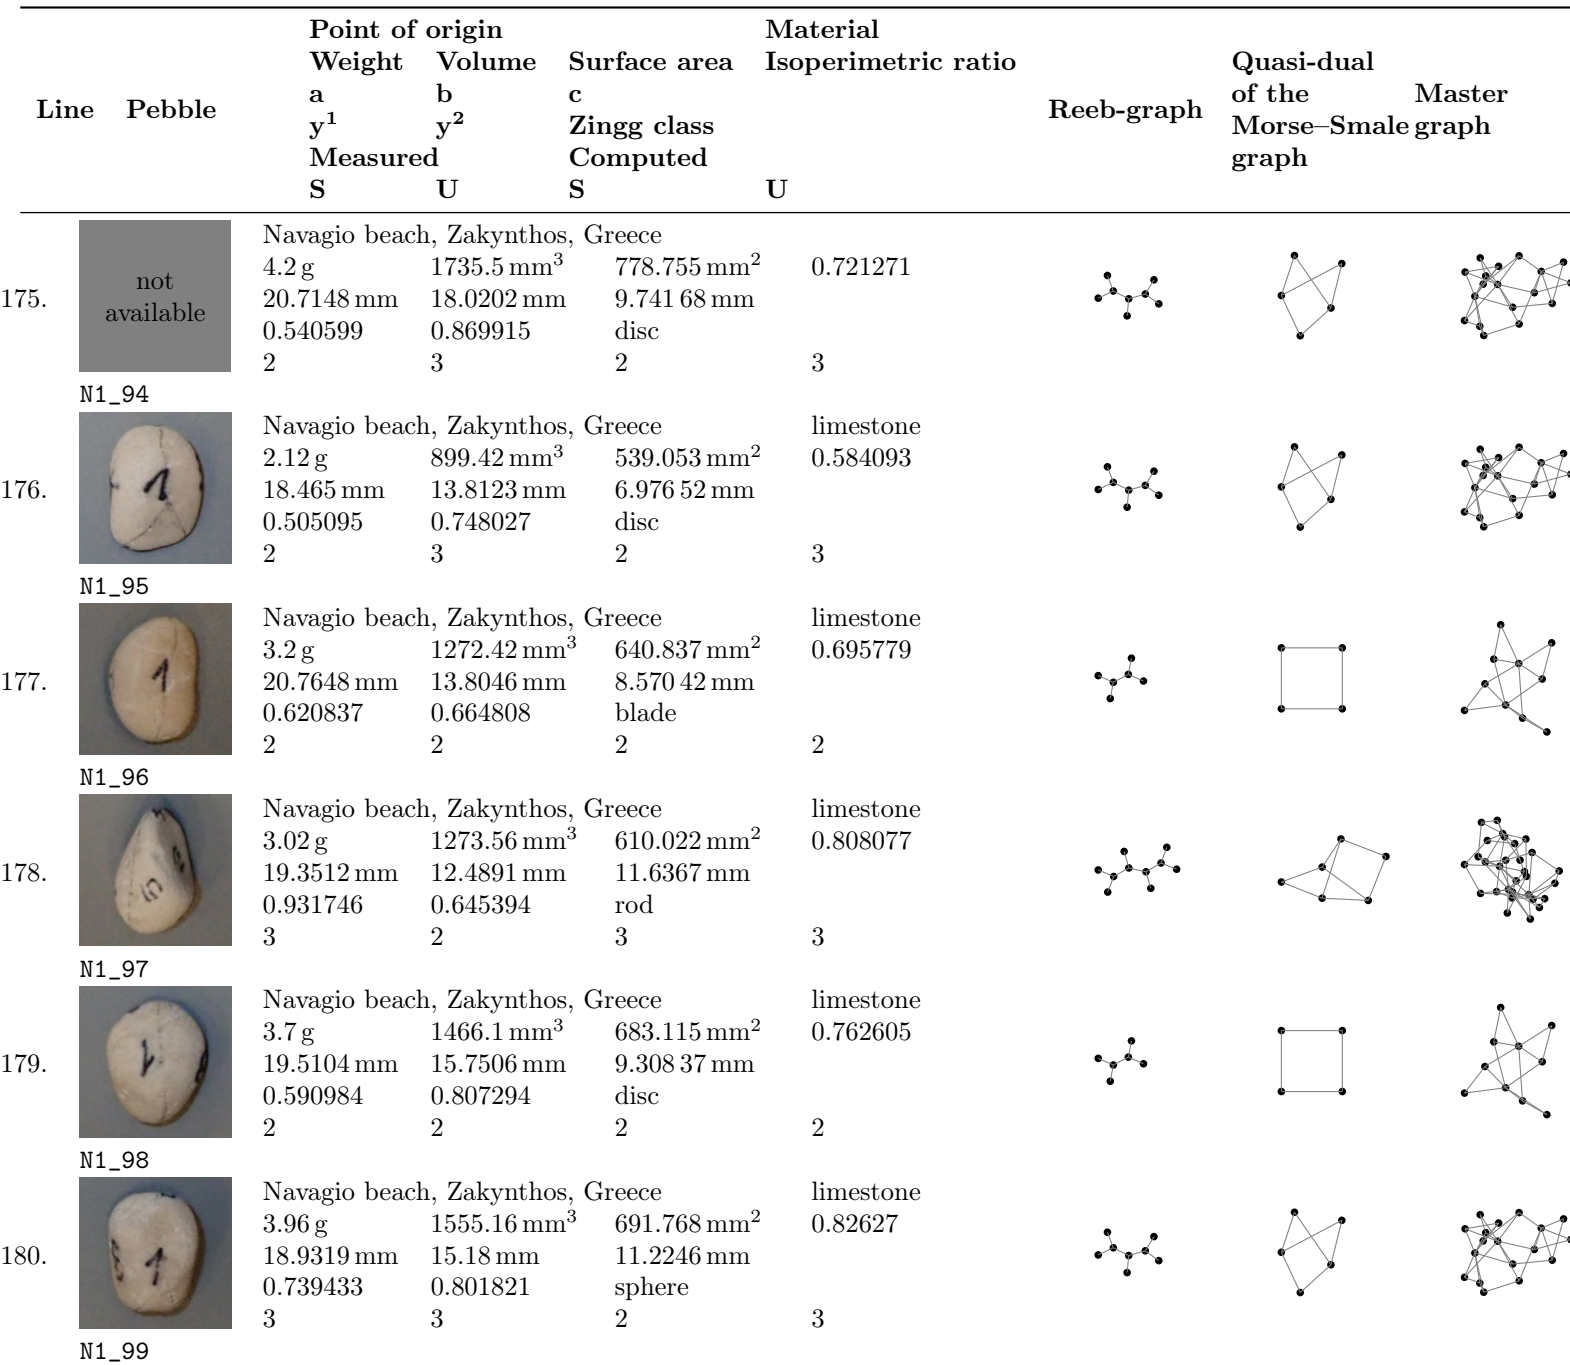   | Navagio beach, Zakynthos, Greece     |                          |                                                   | limestone<br>0.695779                | 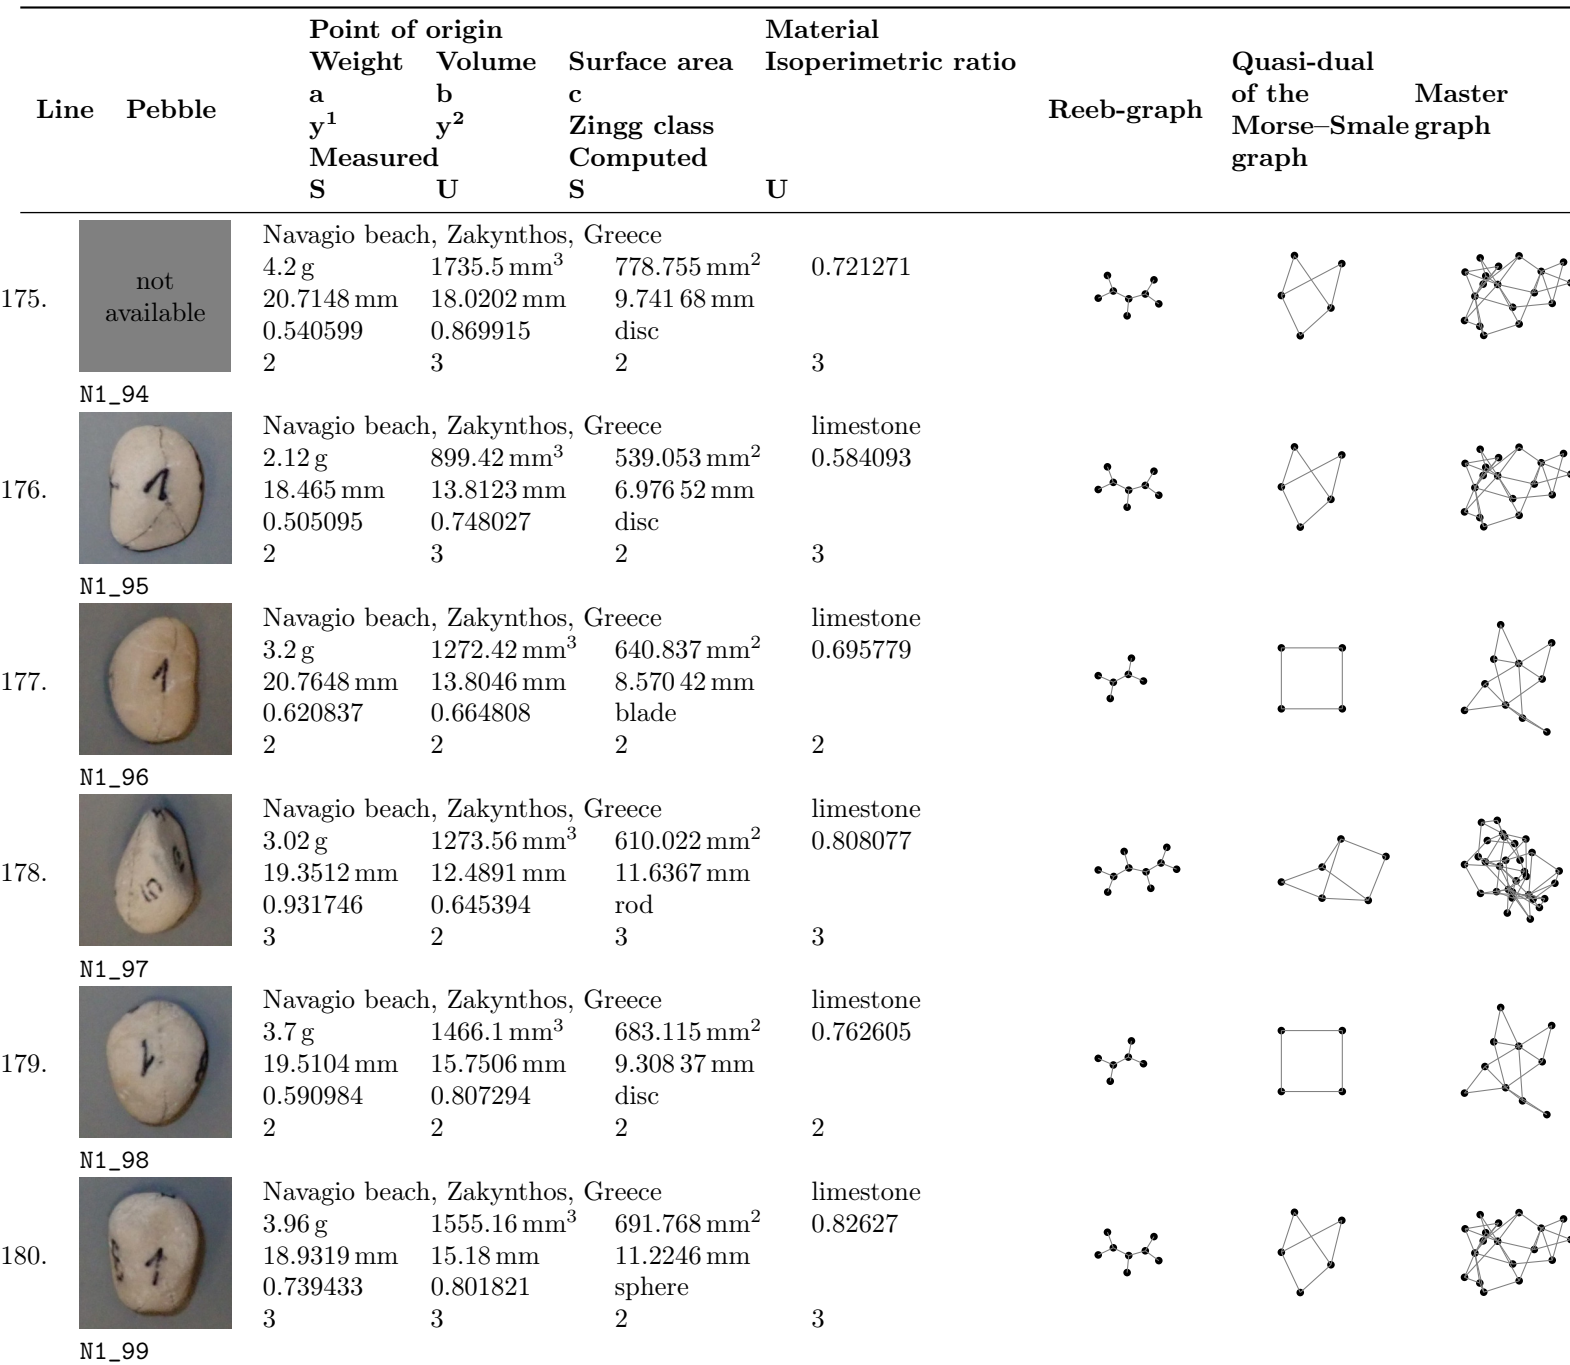   | 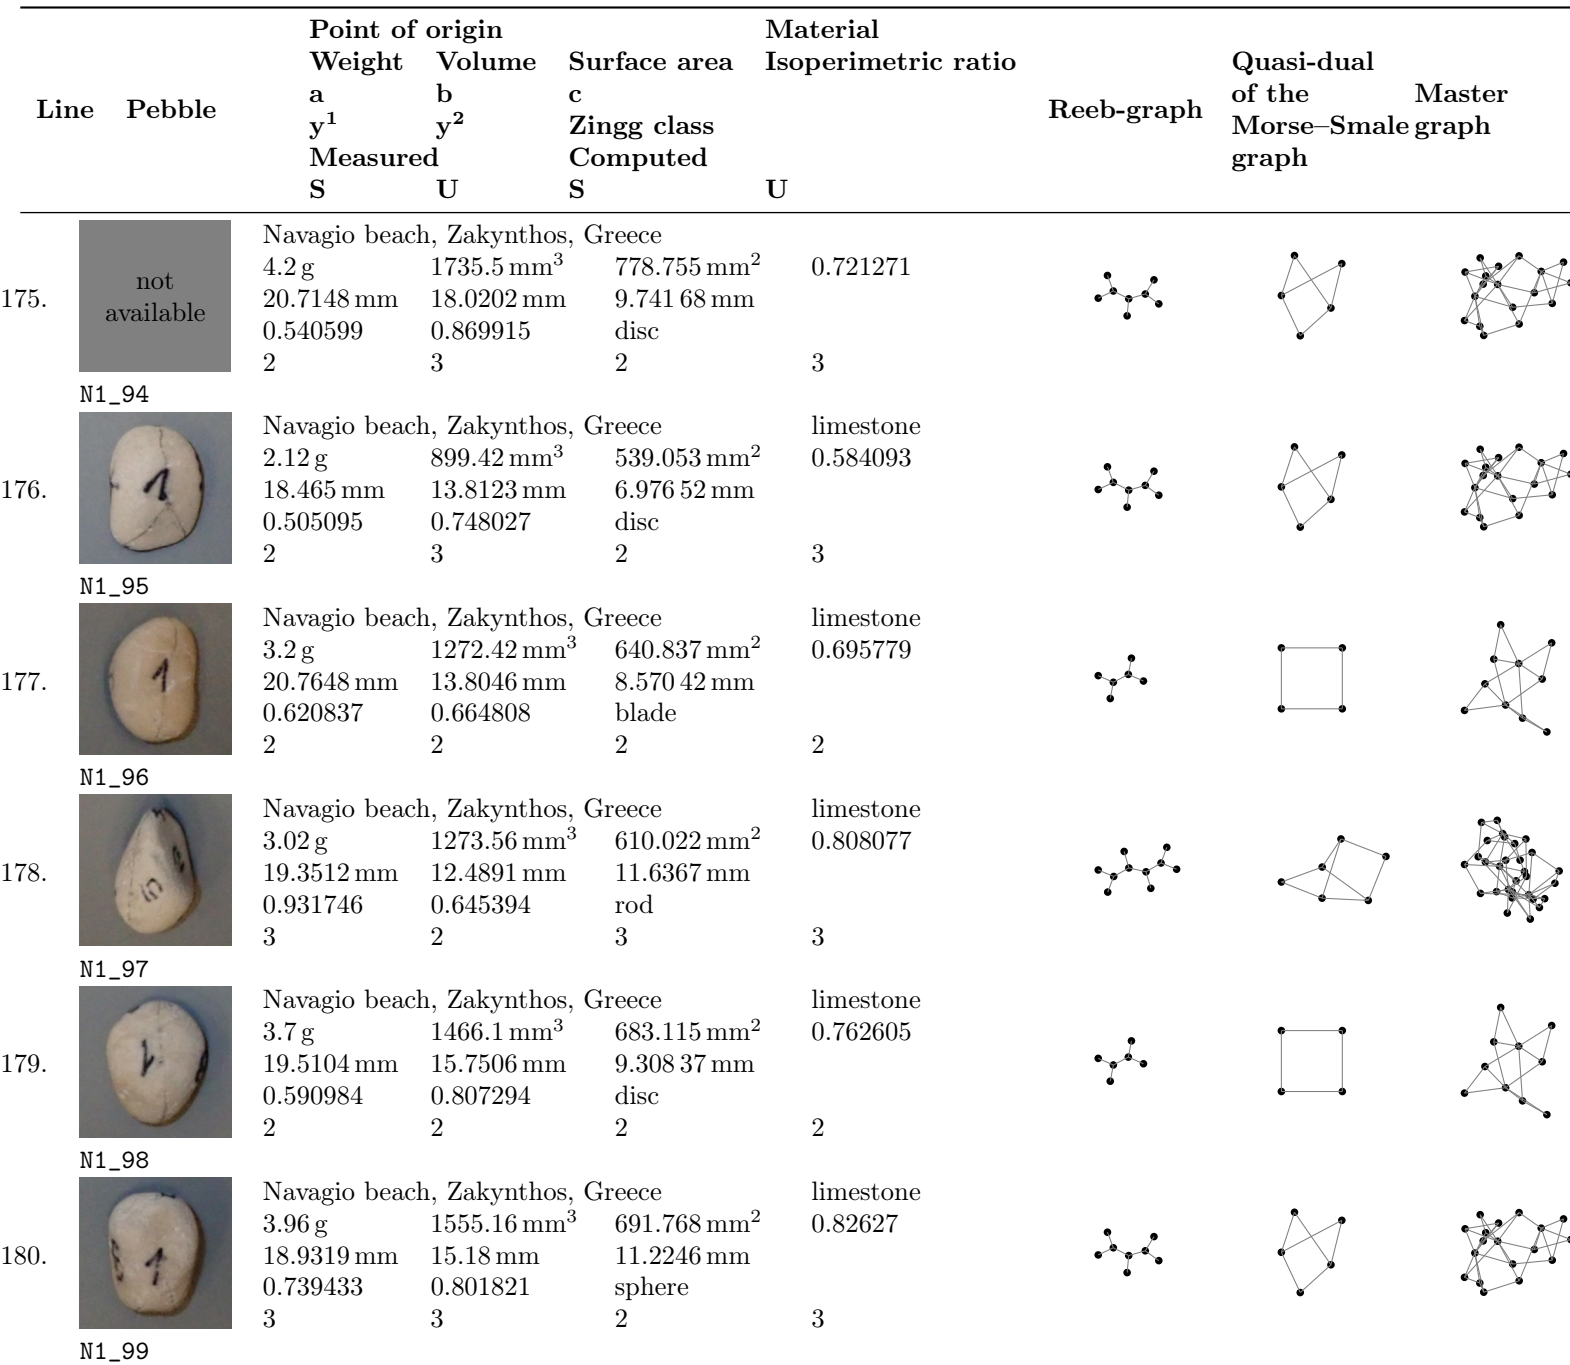   | 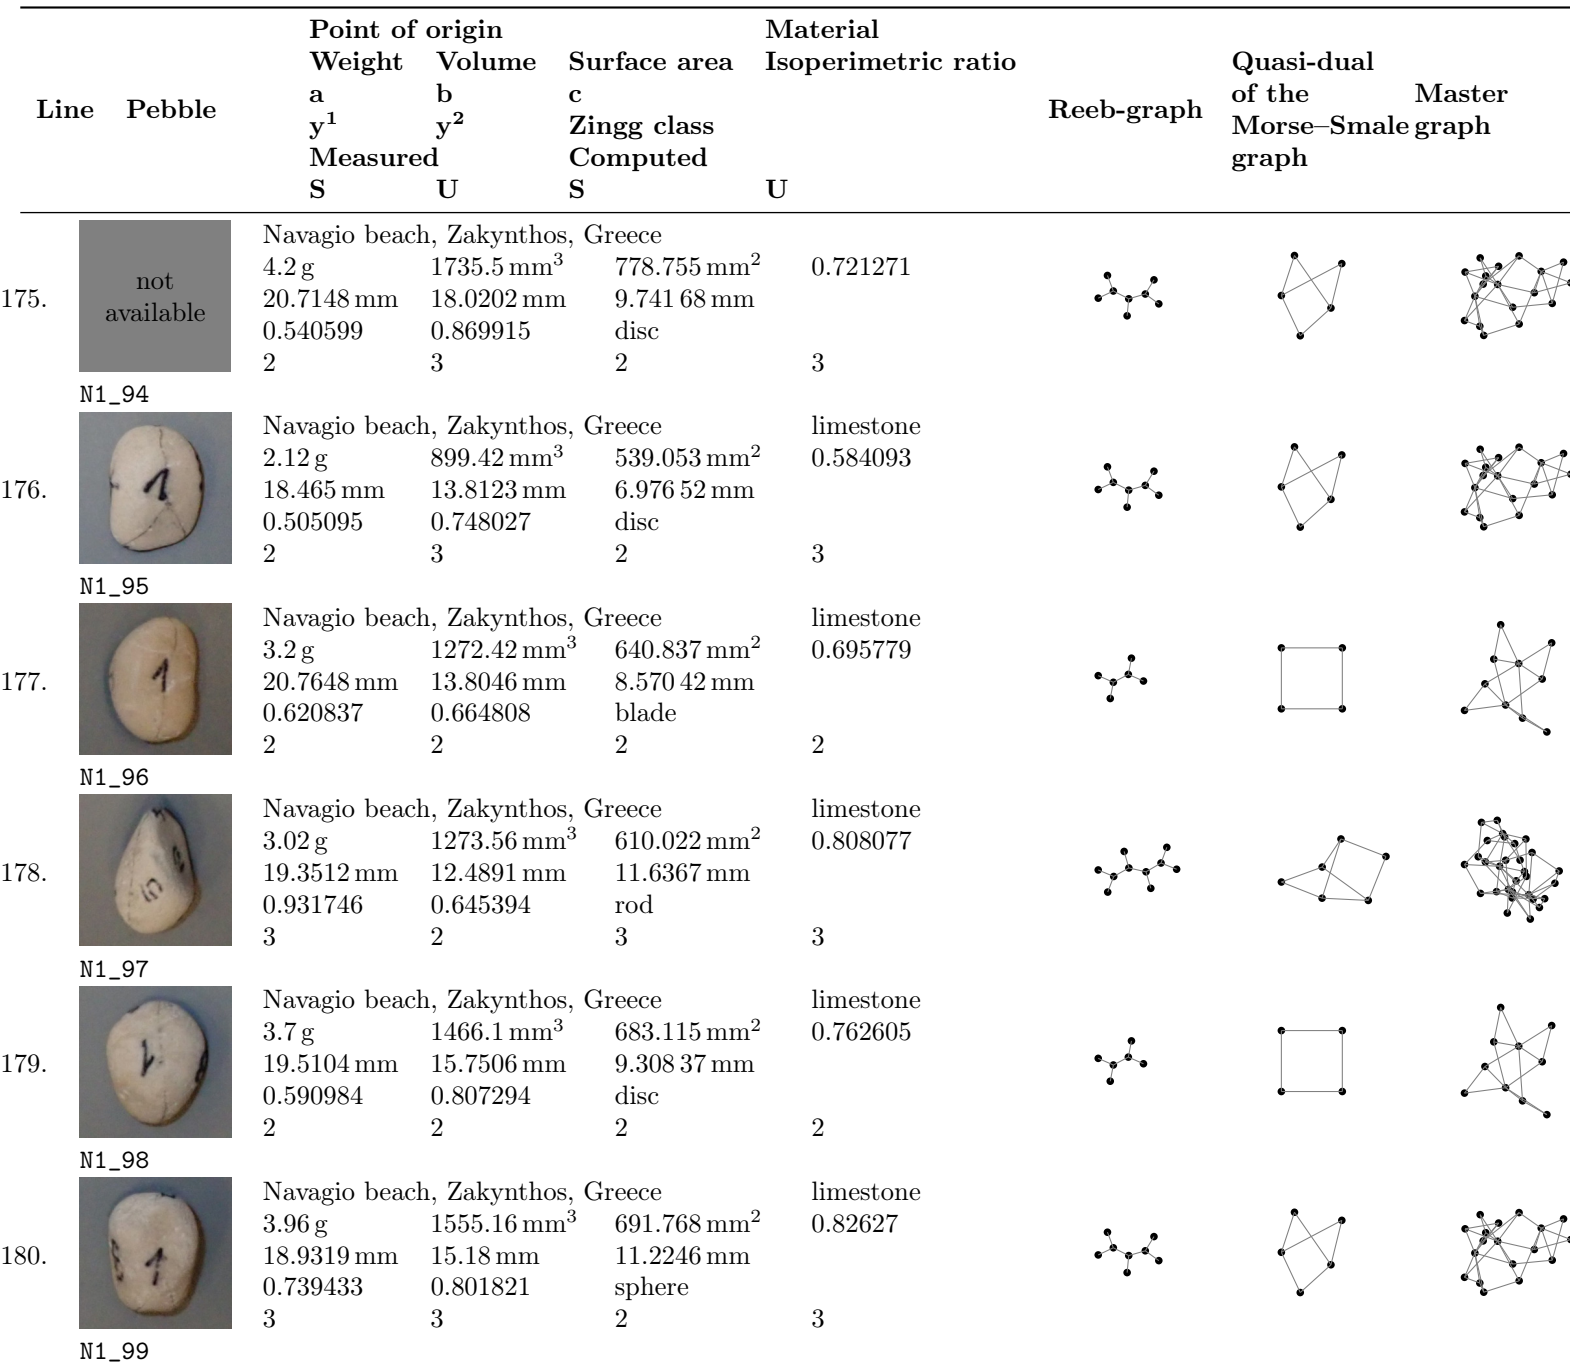   |
|      |                                                                                     | 3.2 g                                | 1272.42 mm <sup>3</sup>  | 640.837 mm <sup>2</sup>                           |                                      |                                                                                       |                                                                                       |                                                                                       |
|      |                                                                                     | 20.7648 mm                           | 13.8046 mm               | 8.570 42 mm                                       |                                      |                                                                                       |                                                                                       |                                                                                       |
|      |                                                                                     | 0.620837                             | 0.664808                 | blade                                             |                                      |                                                                                       |                                                                                       |                                                                                       |
|      |                                                                                     | 2                                    | 2                        | 2                                                 |                                      |                                                                                       |                                                                                       |                                                                                       |
|      | N1_96                                                                               |                                      |                          |                                                   |                                      |                                                                                       |                                                                                       |                                                                                       |
| 178. | 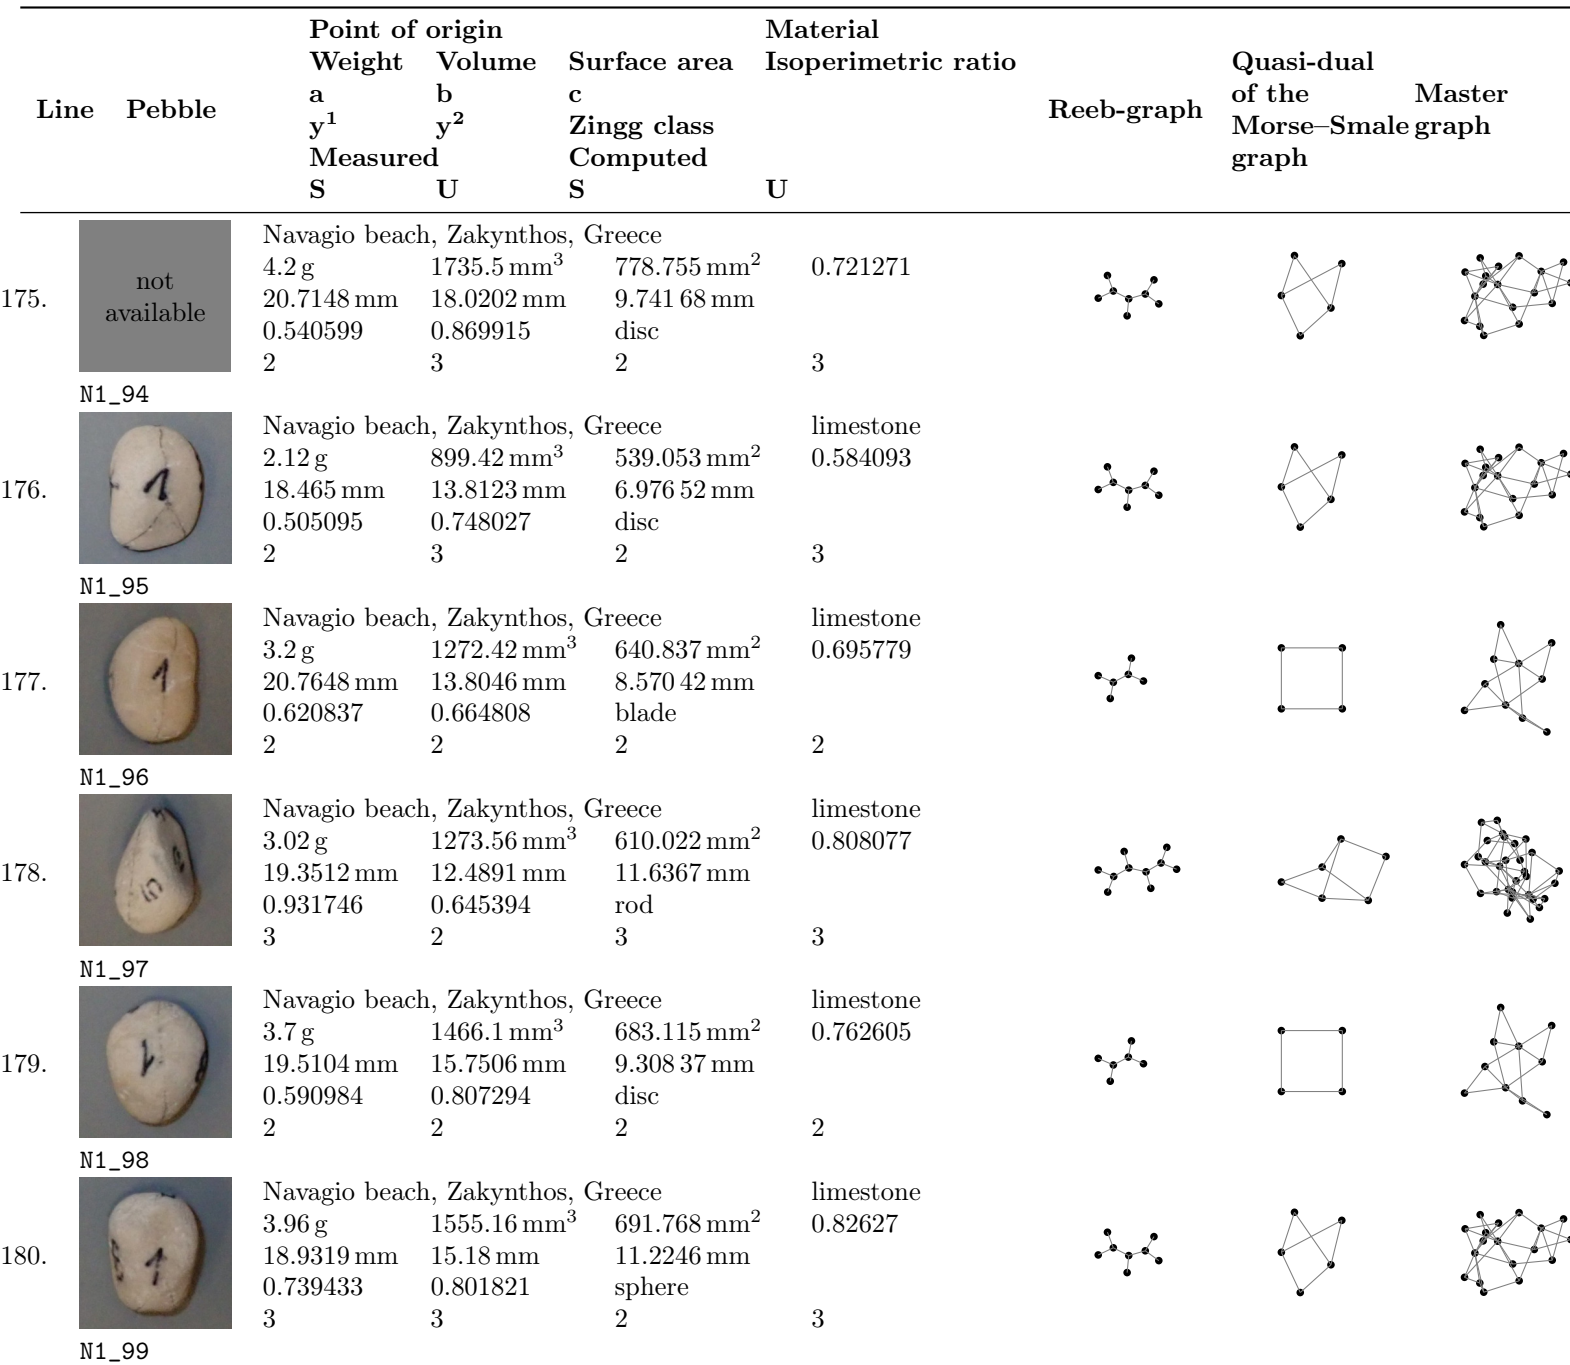  | Navagio beach, Zakynthos, Greece     |                          |                                                   | limestone<br>0.808077                | 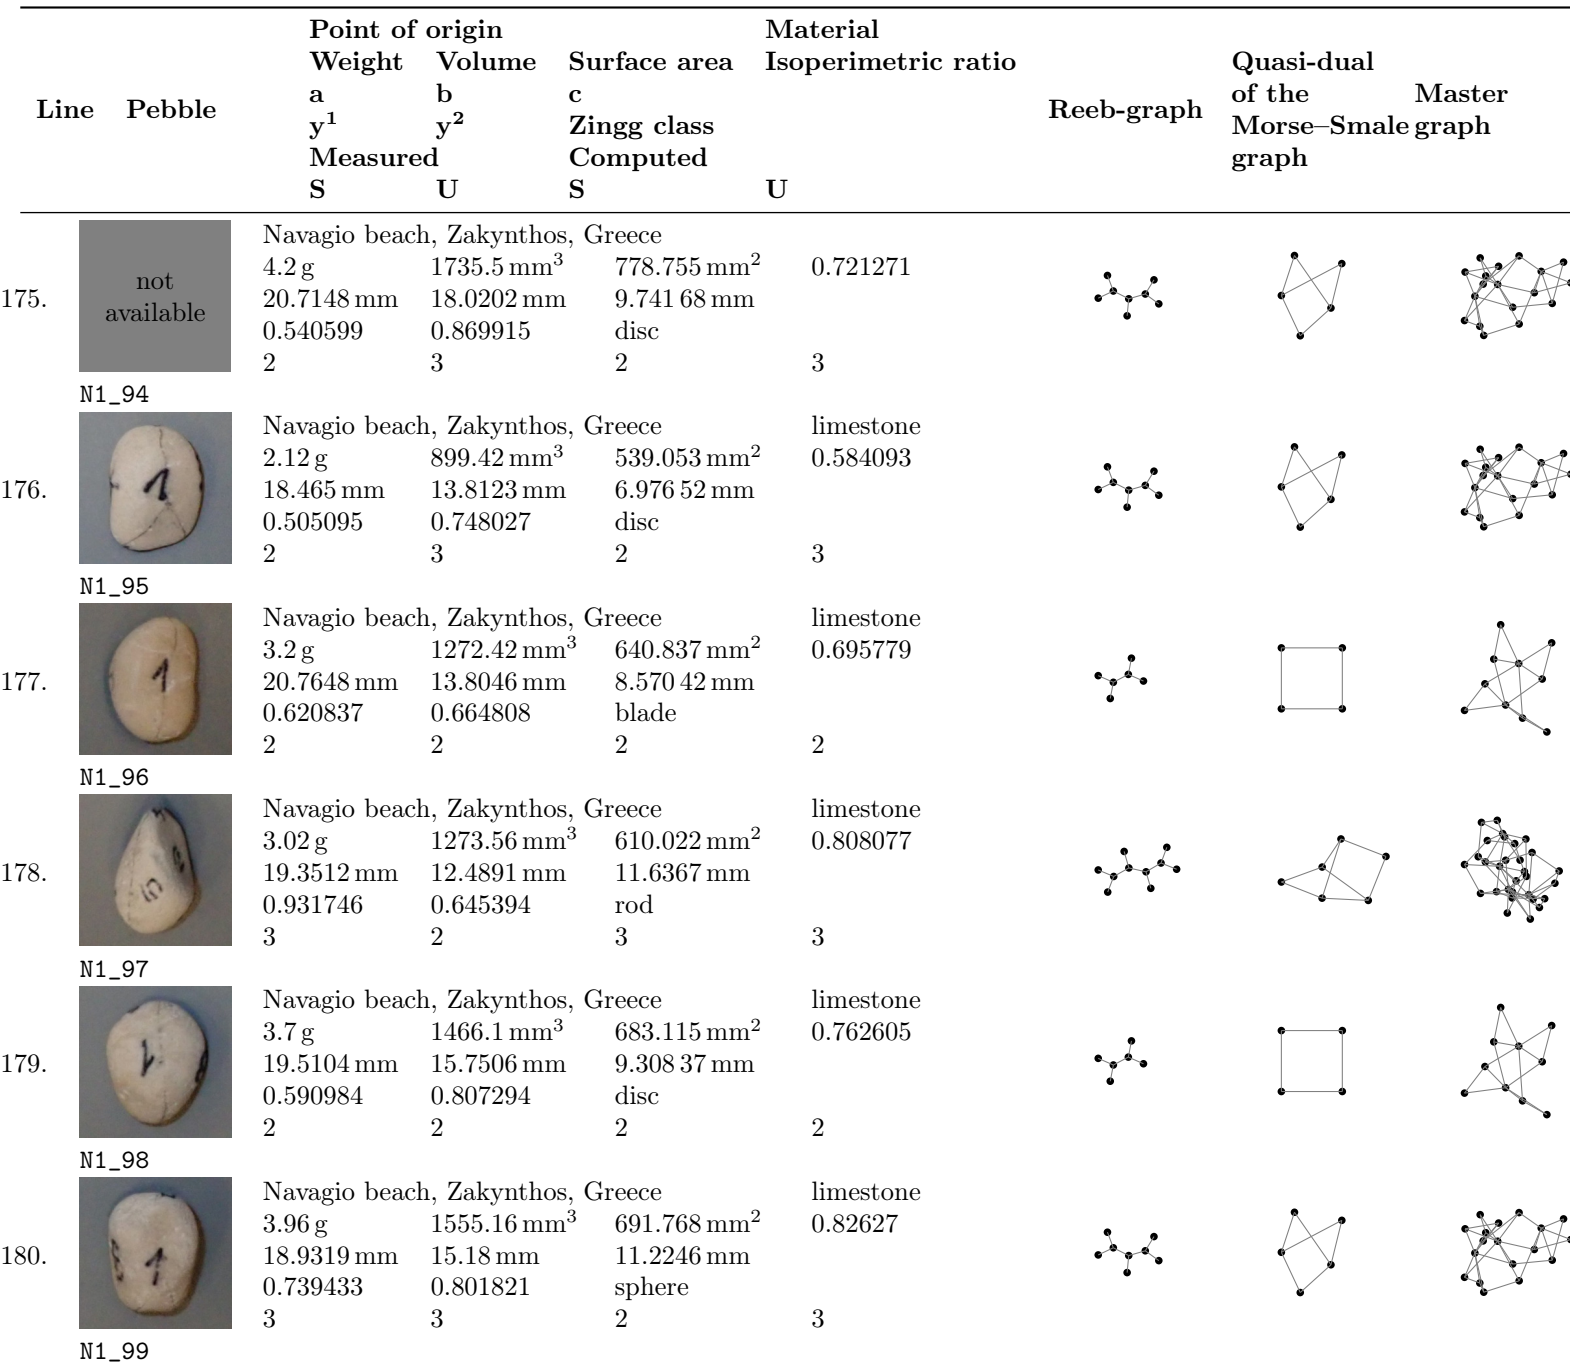  | 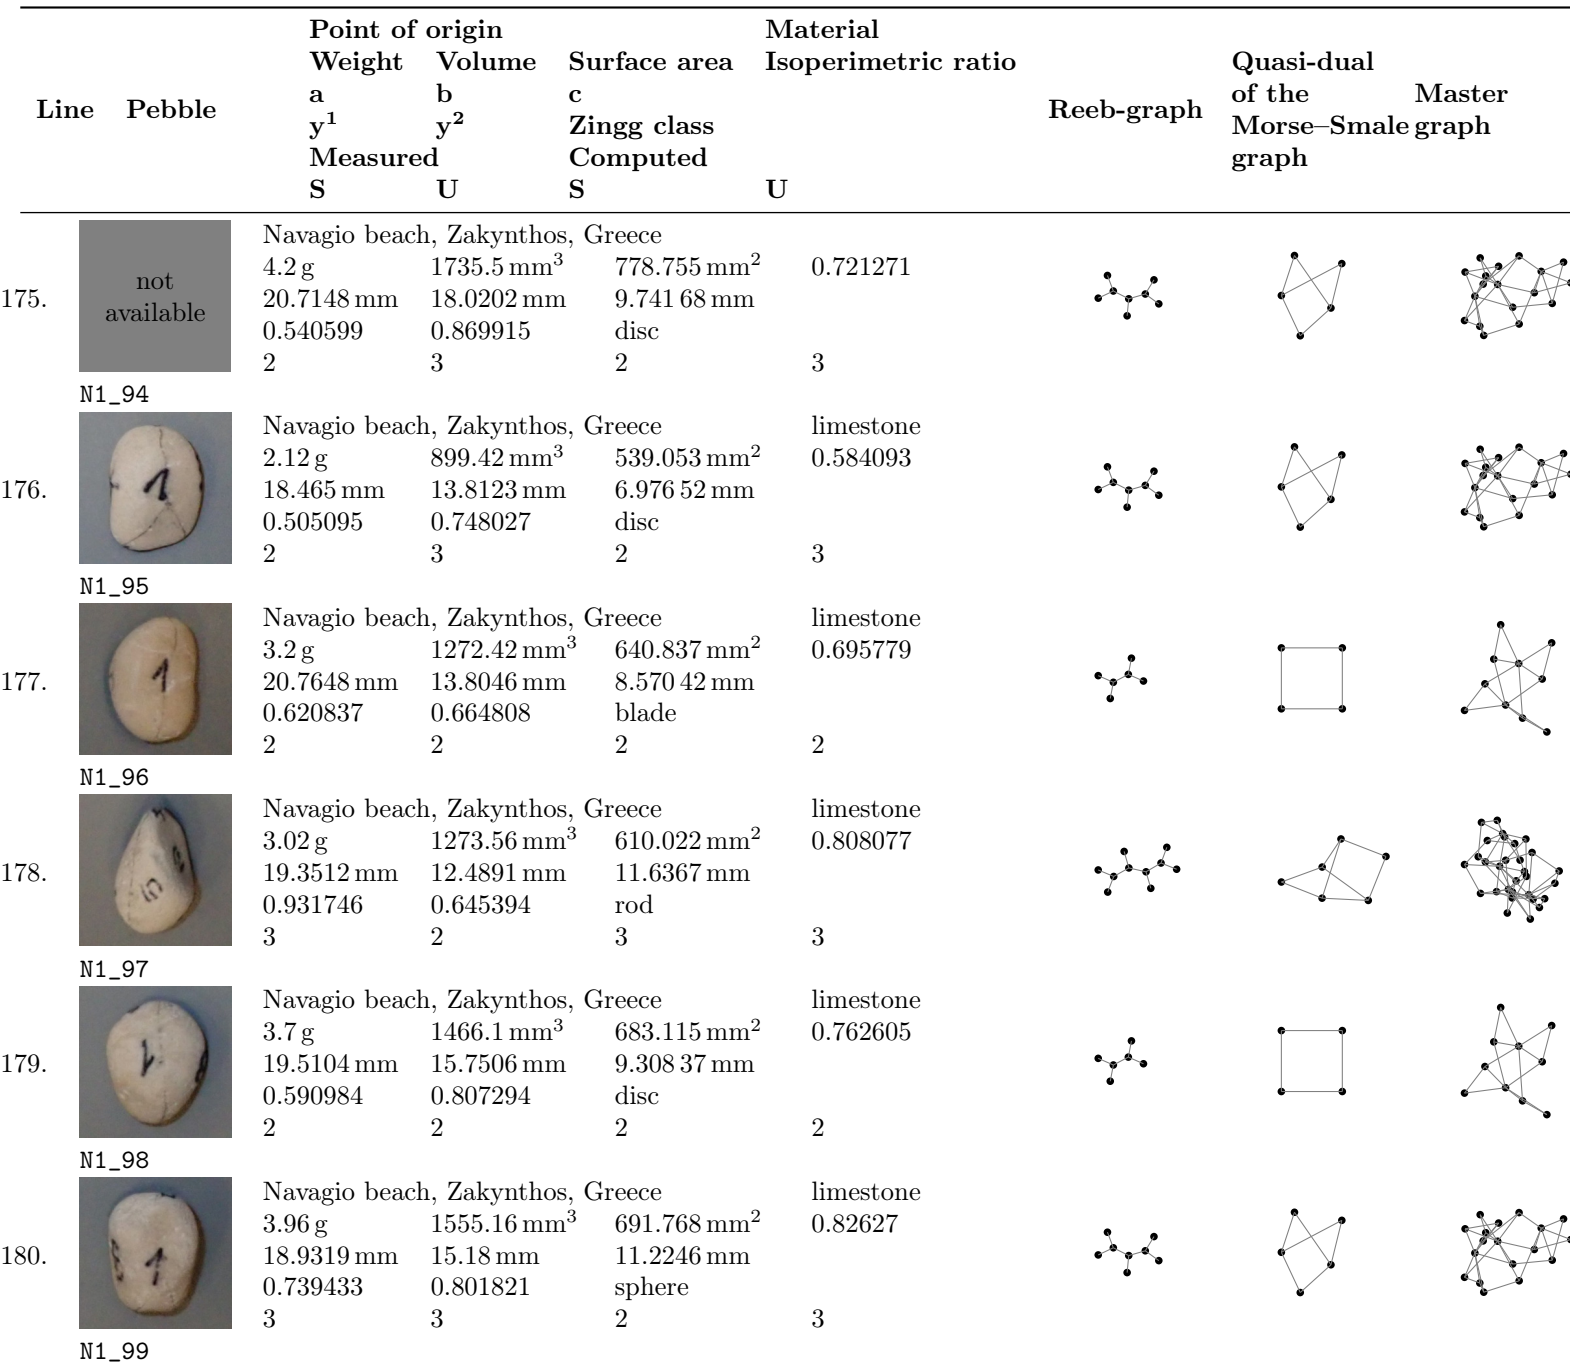  | 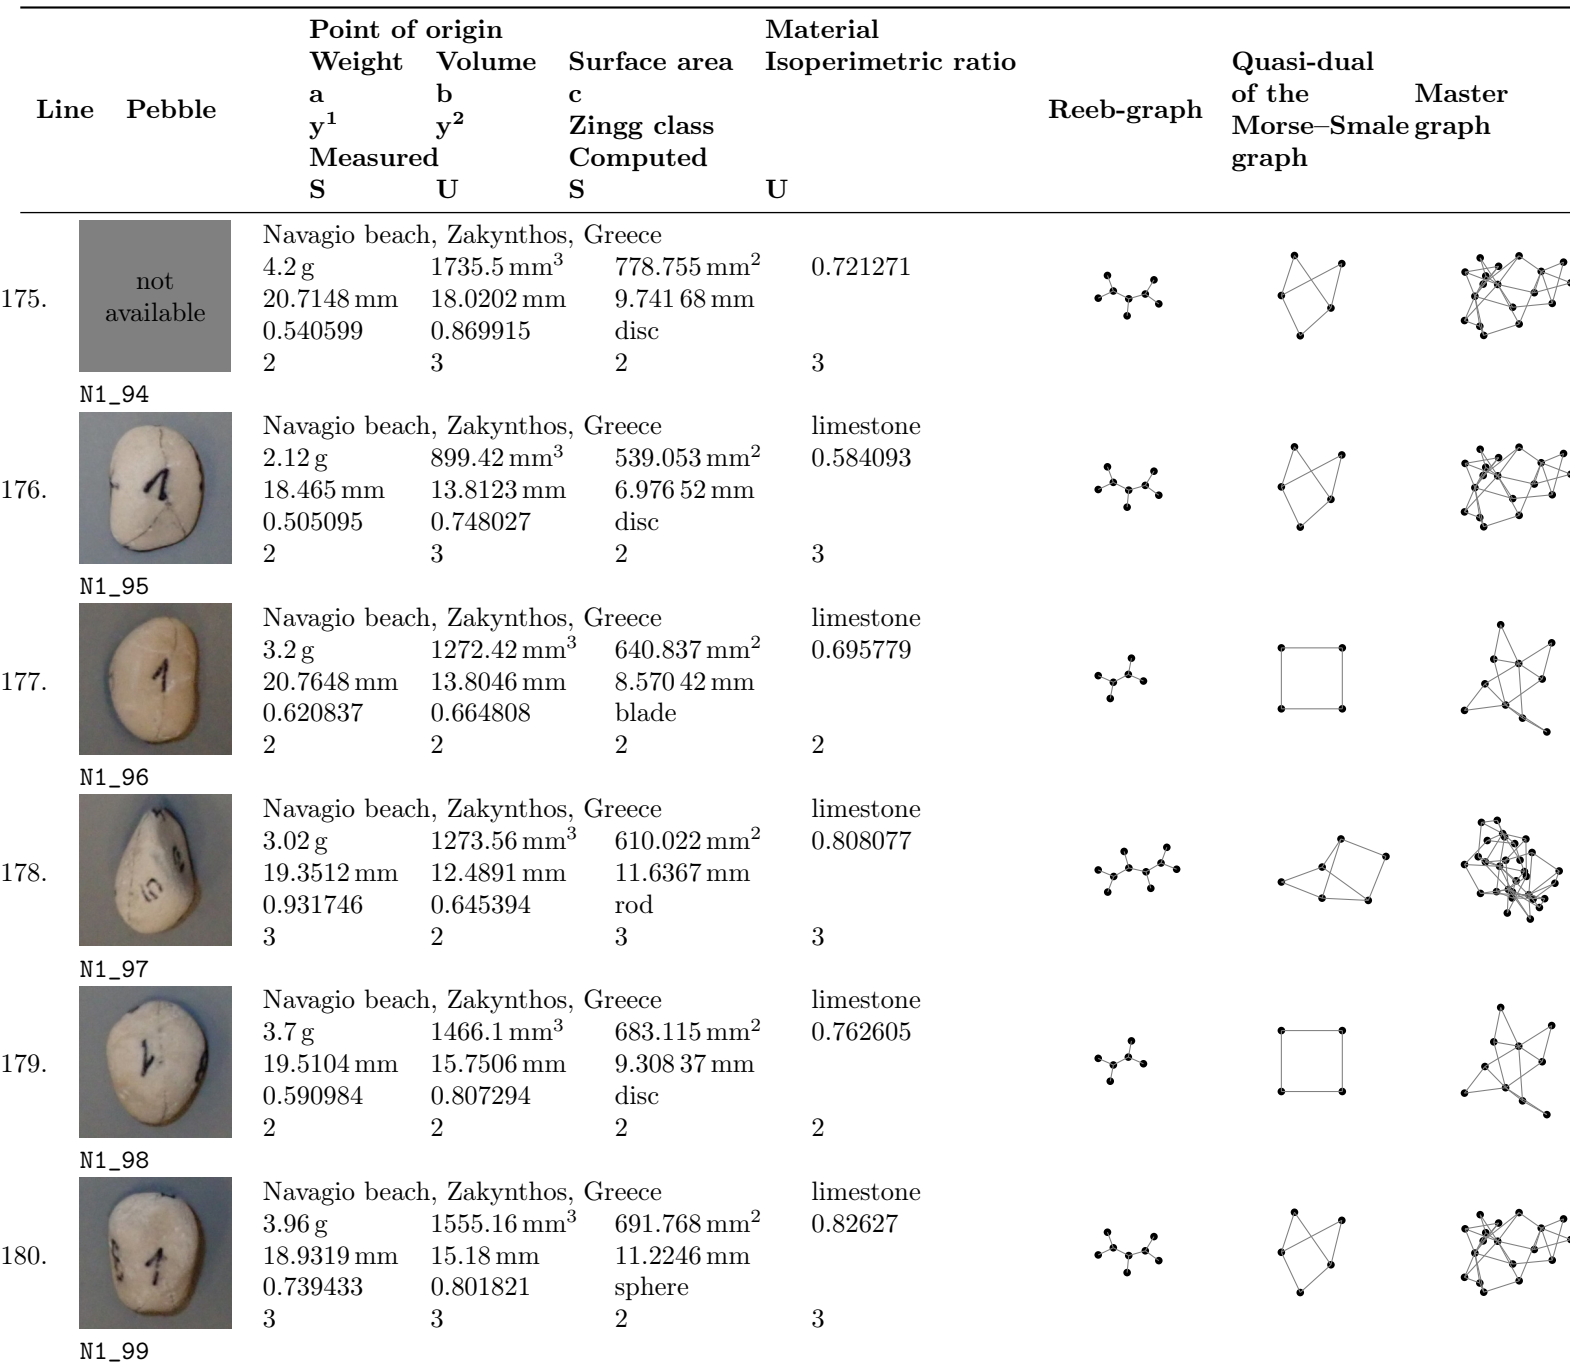  |
|      |                                                                                     | 3.02 g                               | 1273.56 mm <sup>3</sup>  | 610.022 mm <sup>2</sup>                           |                                      |                                                                                       |                                                                                       |                                                                                       |
|      |                                                                                     | 19.3512 mm                           | 12.4891 mm               | 11.6367 mm                                        |                                      |                                                                                       |                                                                                       |                                                                                       |
|      |                                                                                     | 0.931746                             | 0.645394                 | rod                                               |                                      |                                                                                       |                                                                                       |                                                                                       |
|      |                                                                                     | 3                                    | 2                        | 3                                                 |                                      |                                                                                       |                                                                                       |                                                                                       |
|      | N1_97                                                                               |                                      |                          |                                                   |                                      |                                                                                       |                                                                                       |                                                                                       |
| 179. | 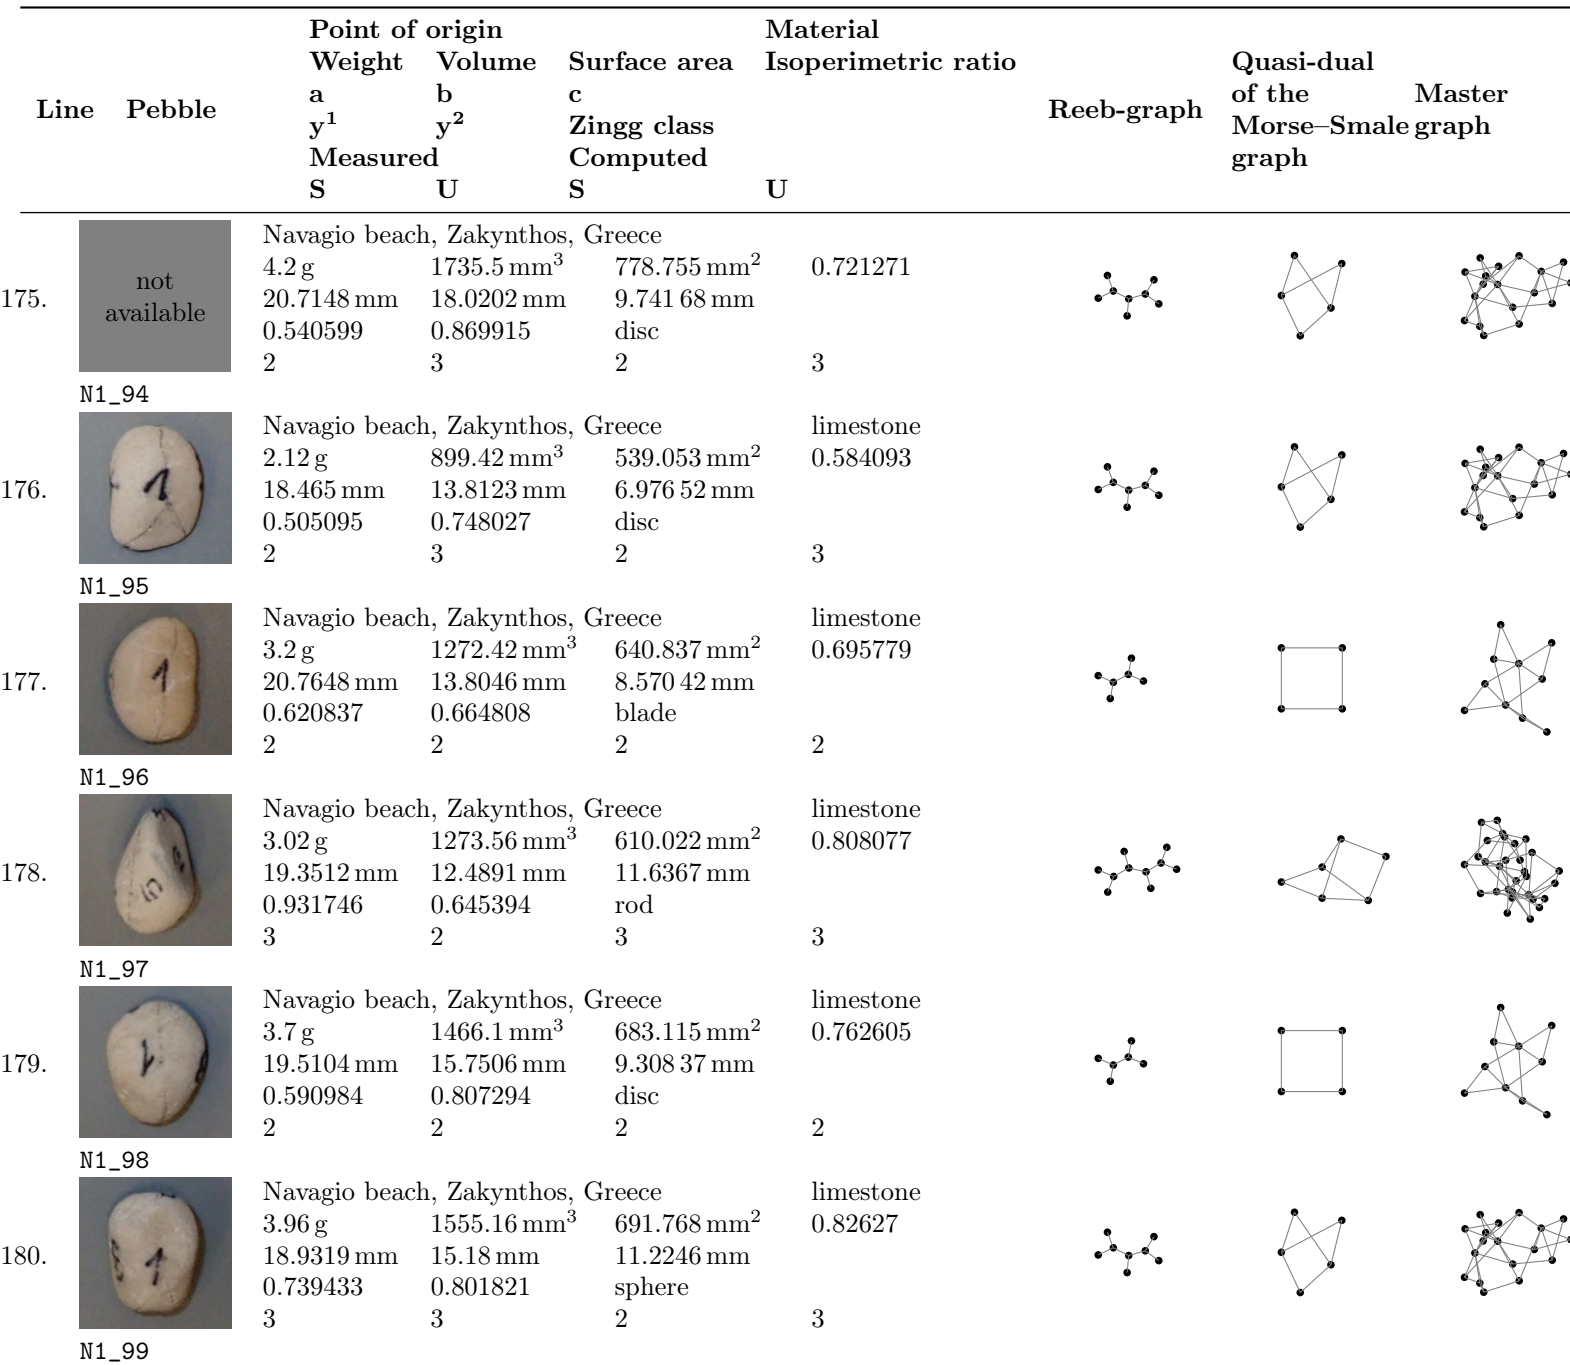 | Navagio beach, Zakynthos, Greece     |                          |                                                   | limestone<br>0.762605                | 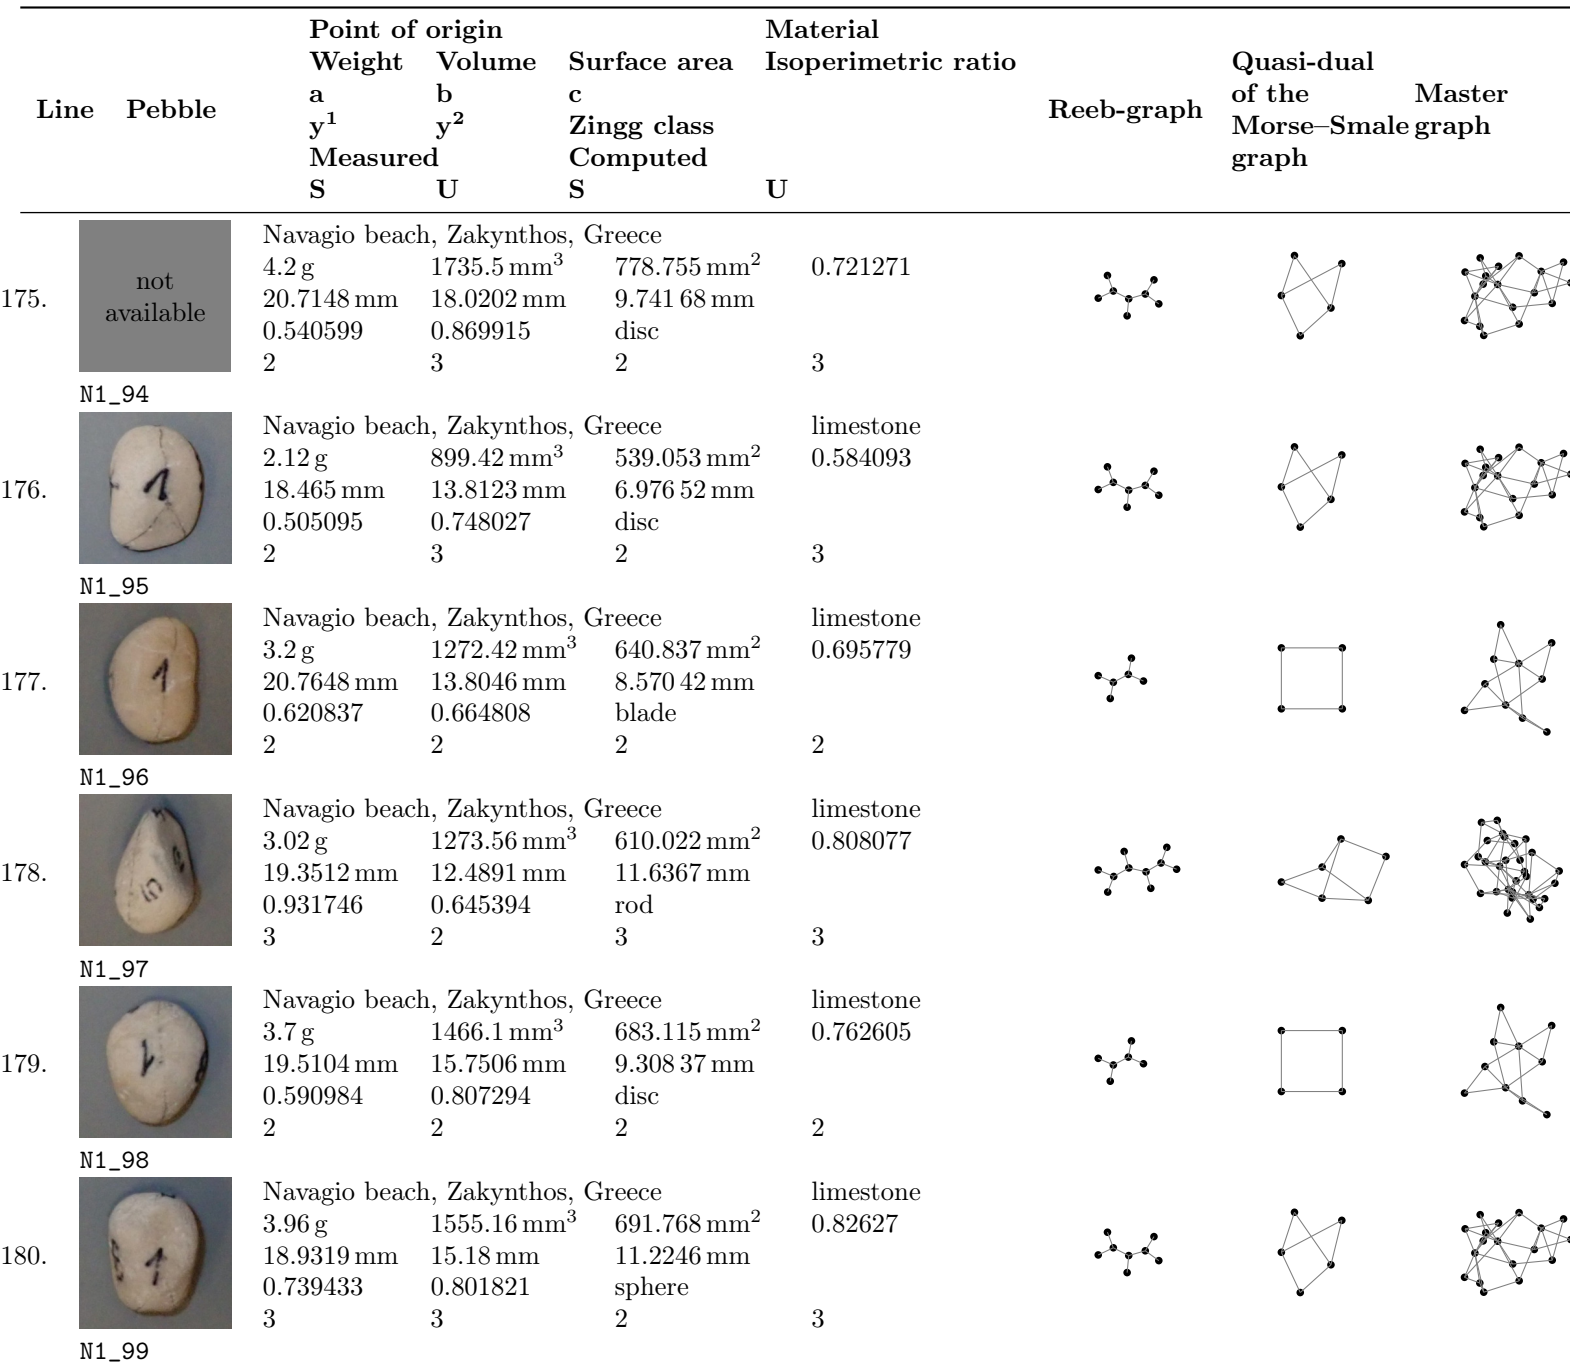 | 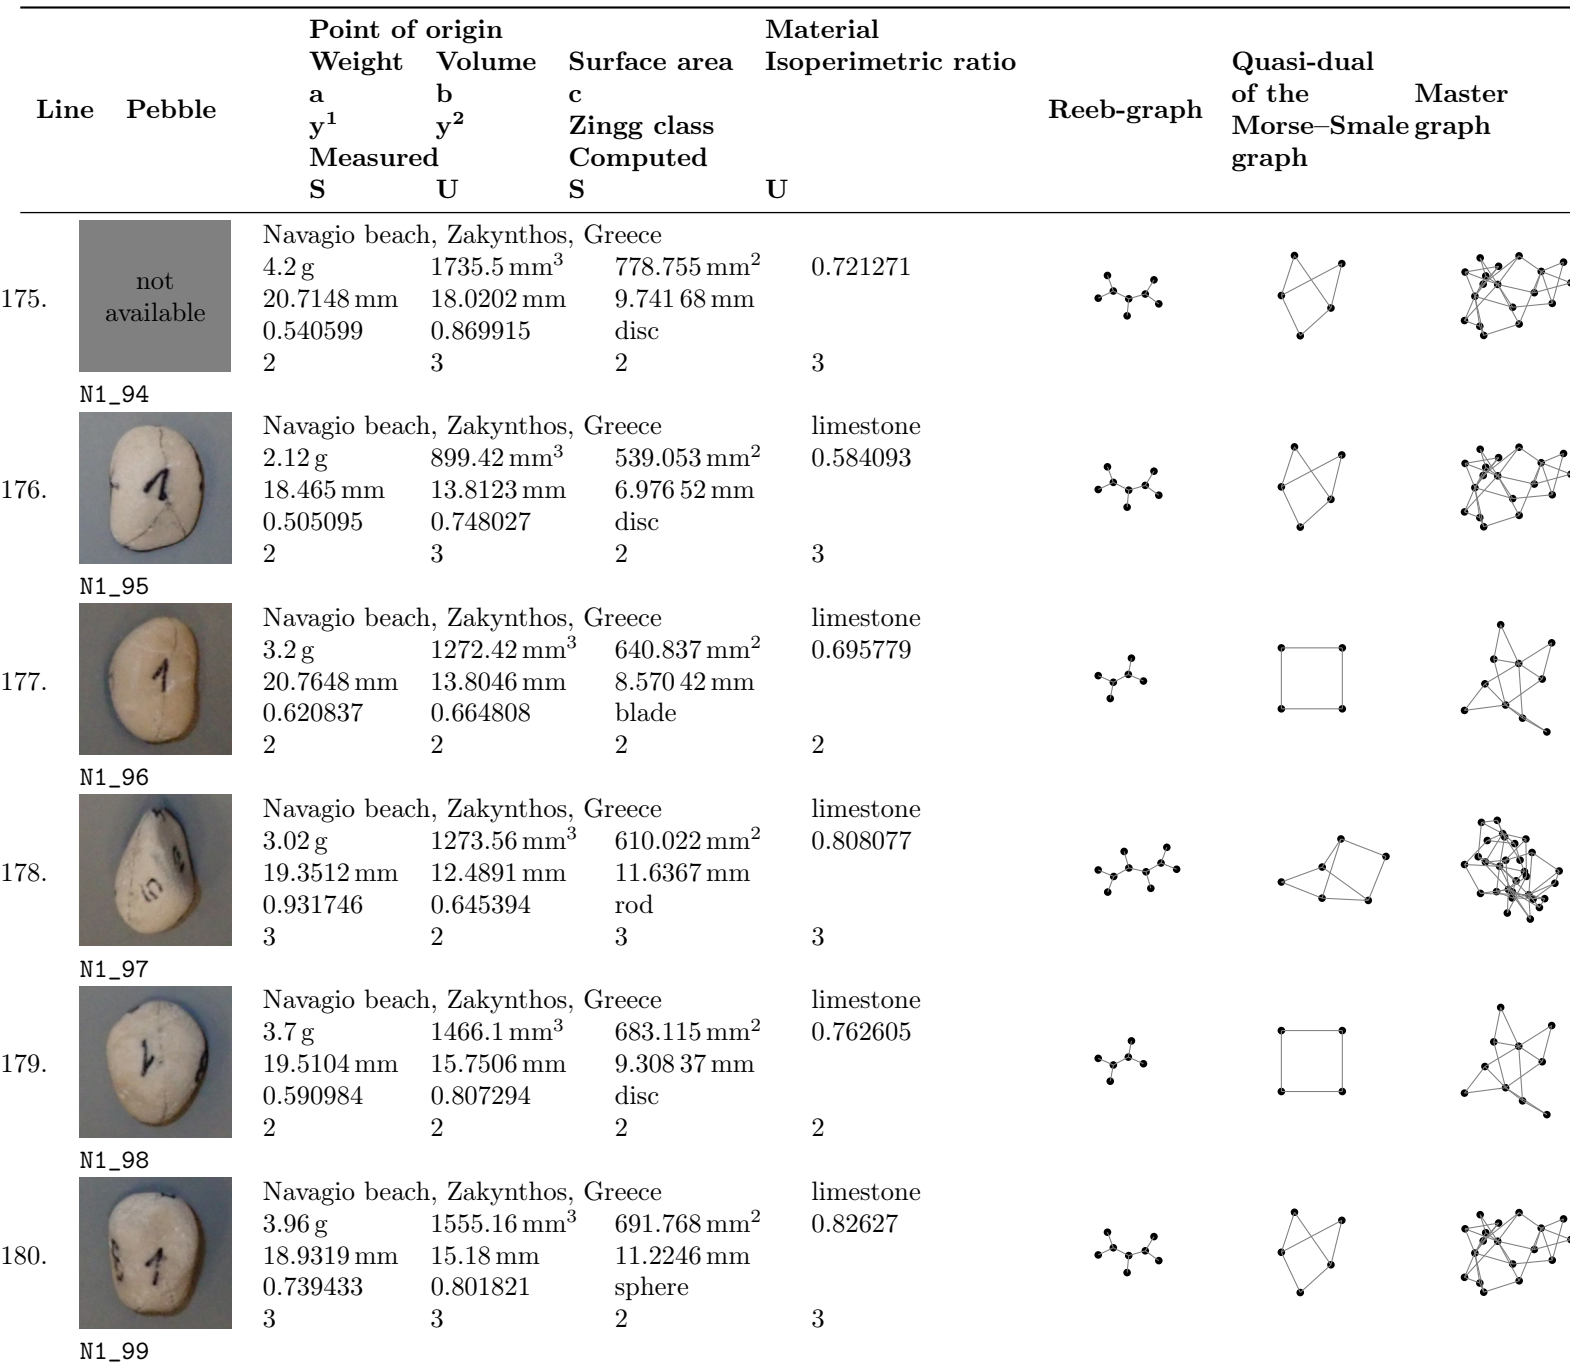 | 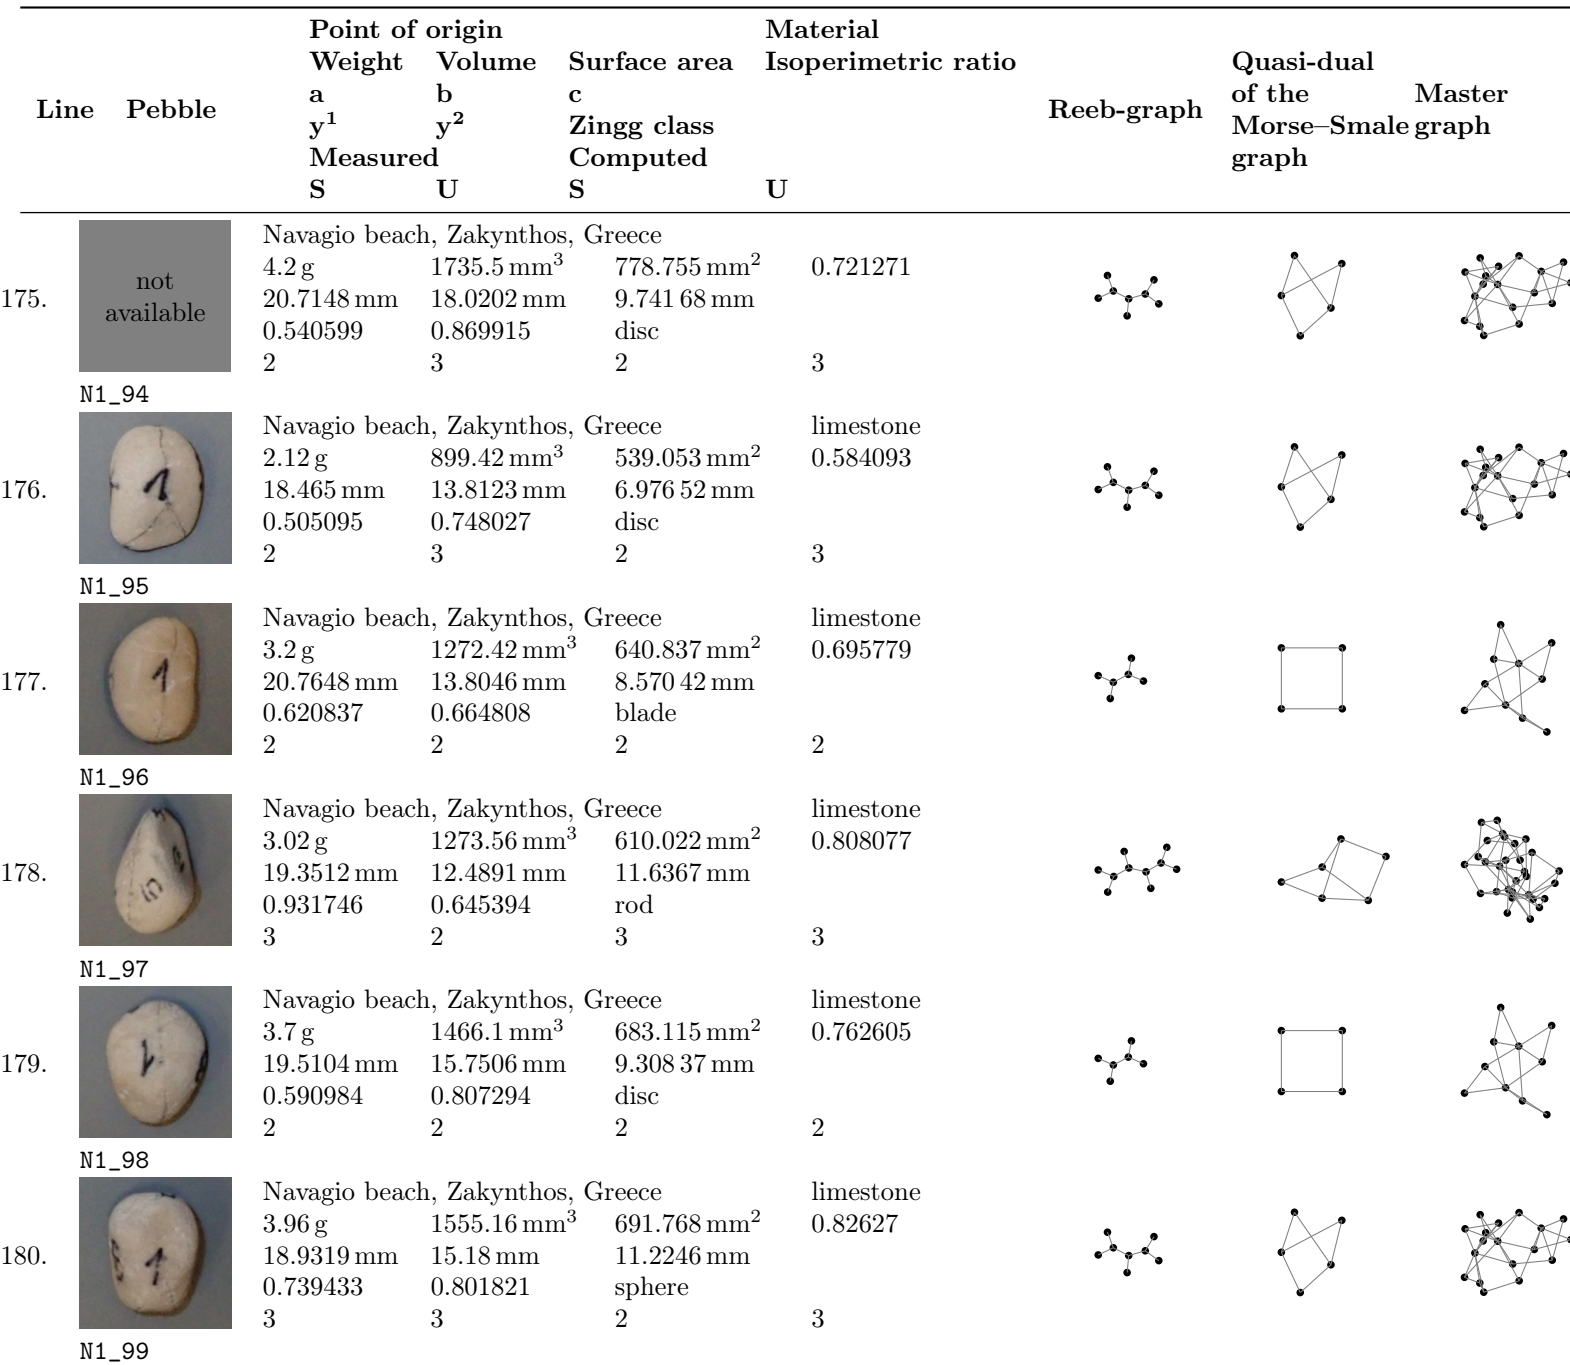 |
|      |                                                                                     | 3.7 g                                | 1466.1 mm <sup>3</sup>   | 683.115 mm <sup>2</sup>                           |                                      |                                                                                       |                                                                                       |                                                                                       |
|      |                                                                                     | 19.5104 mm                           | 15.7506 mm               | 9.308 37 mm                                       |                                      |                                                                                       |                                                                                       |                                                                                       |
|      |                                                                                     | 0.590984                             | 0.807294                 | disc                                              |                                      |                                                                                       |                                                                                       |                                                                                       |
|      |                                                                                     | 2                                    | 2                        | 2                                                 |                                      |                                                                                       |                                                                                       |                                                                                       |
|      | N1_98                                                                               |                                      |                          |                                                   |                                      |                                                                                       |                                                                                       |                                                                                       |
| 180. | 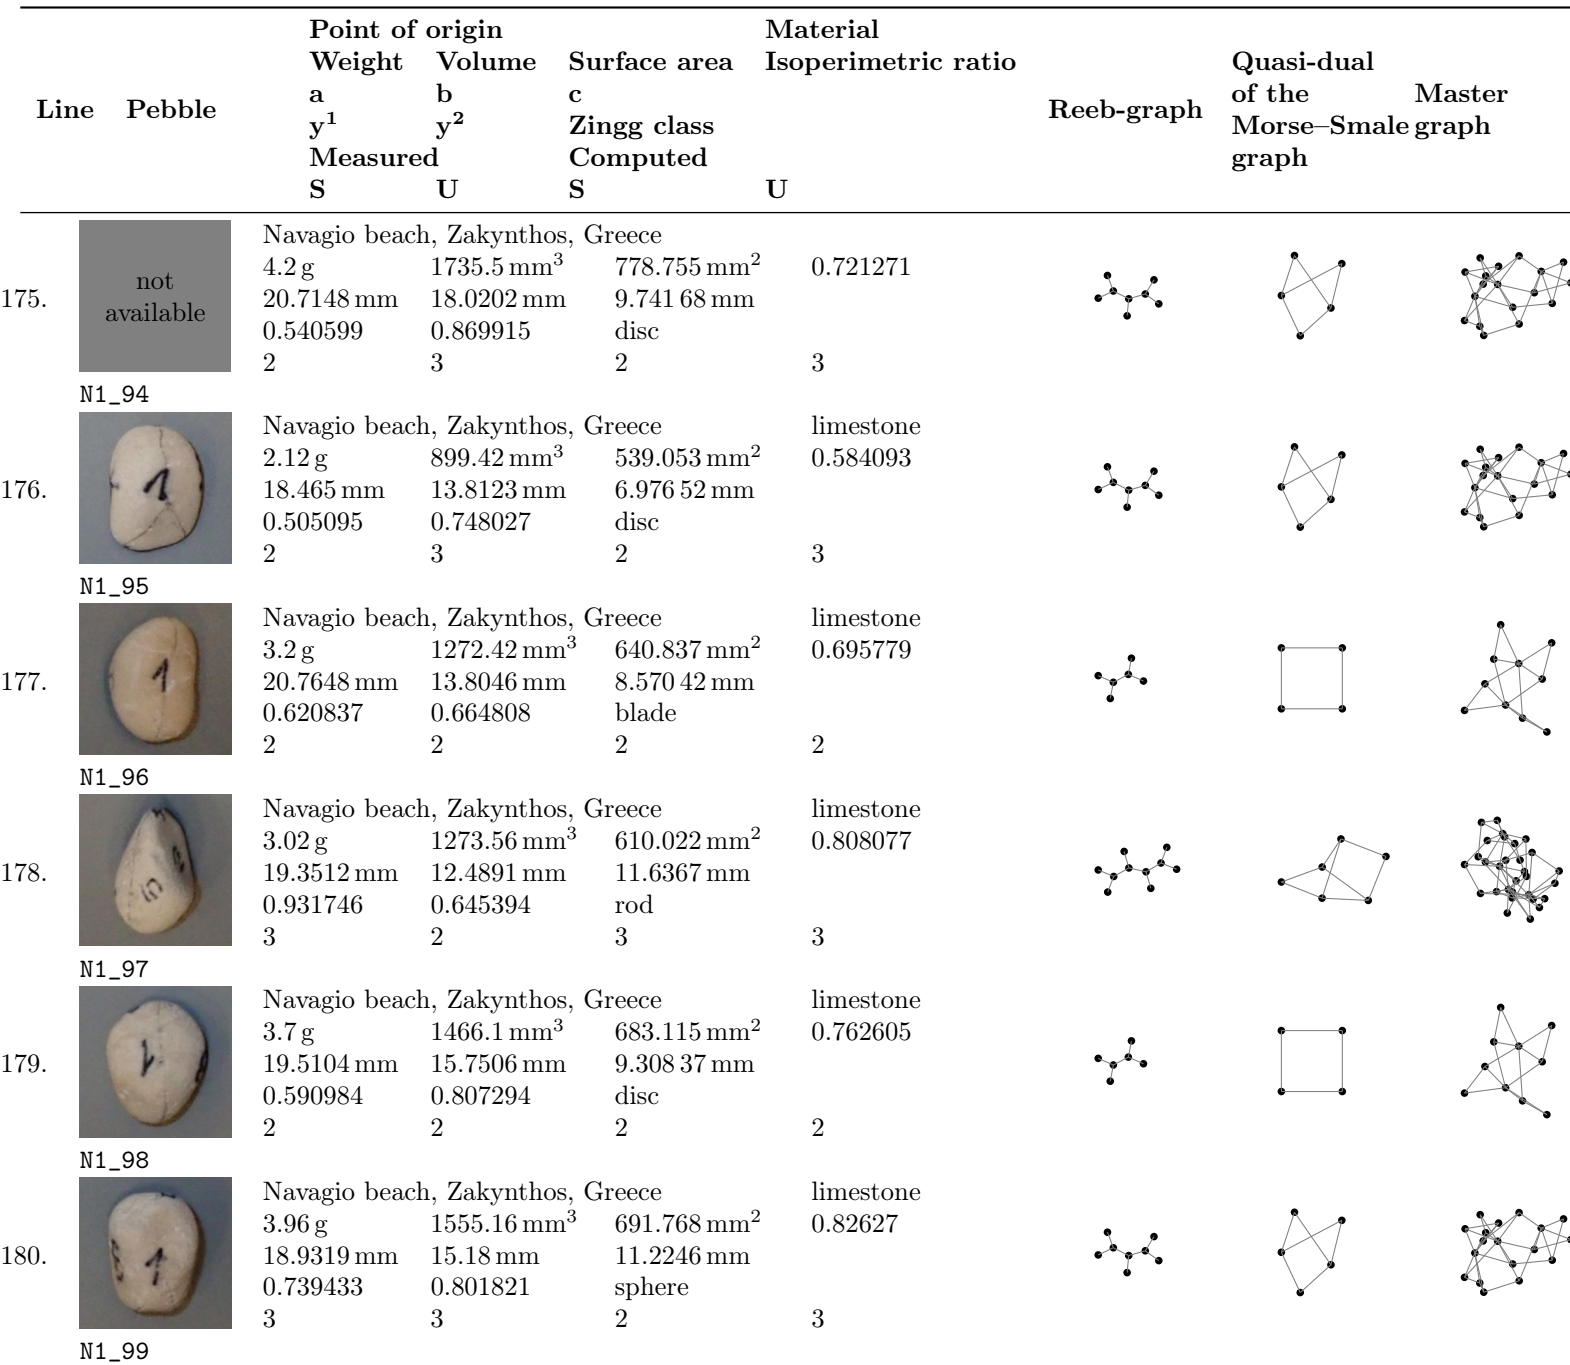 | Navagio beach, Zakynthos, Greece     |                          |                                                   | limestone<br>0.82627                 | 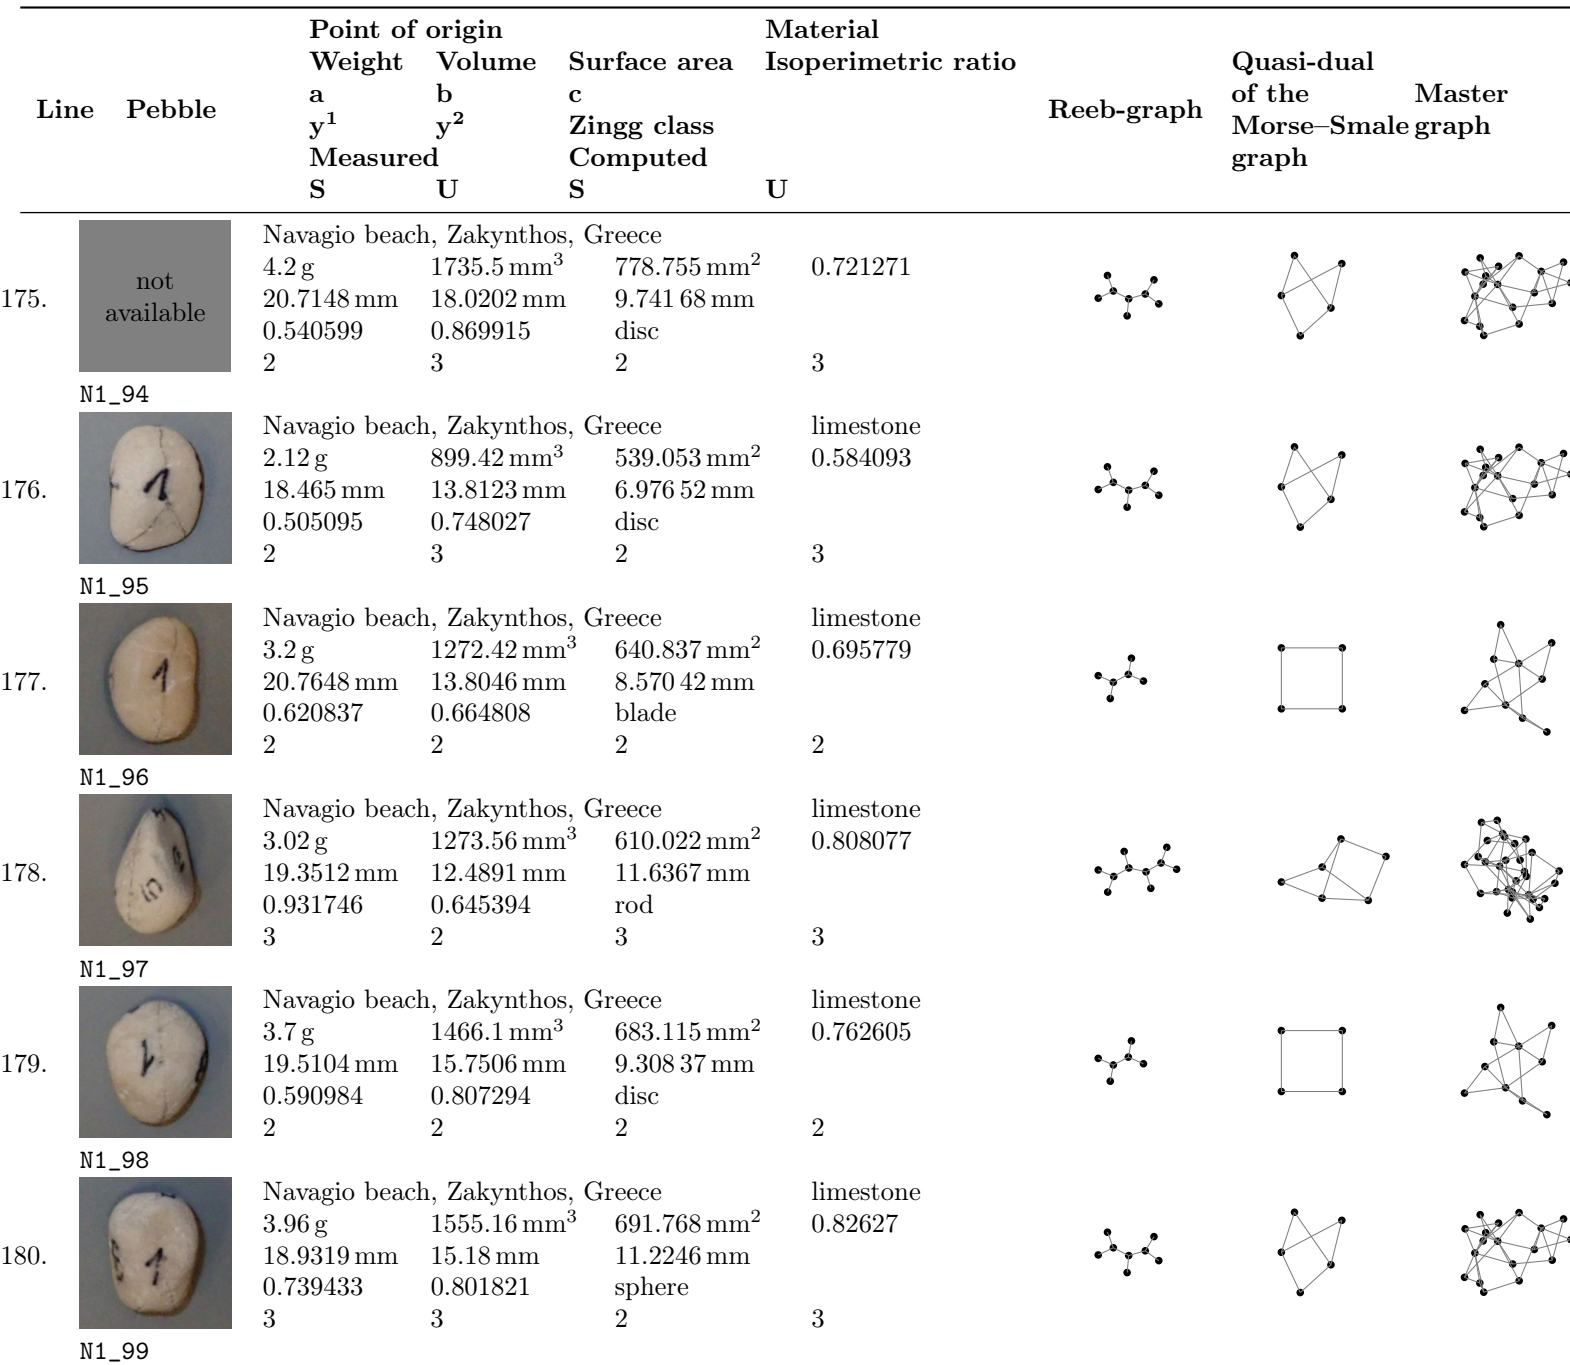 | 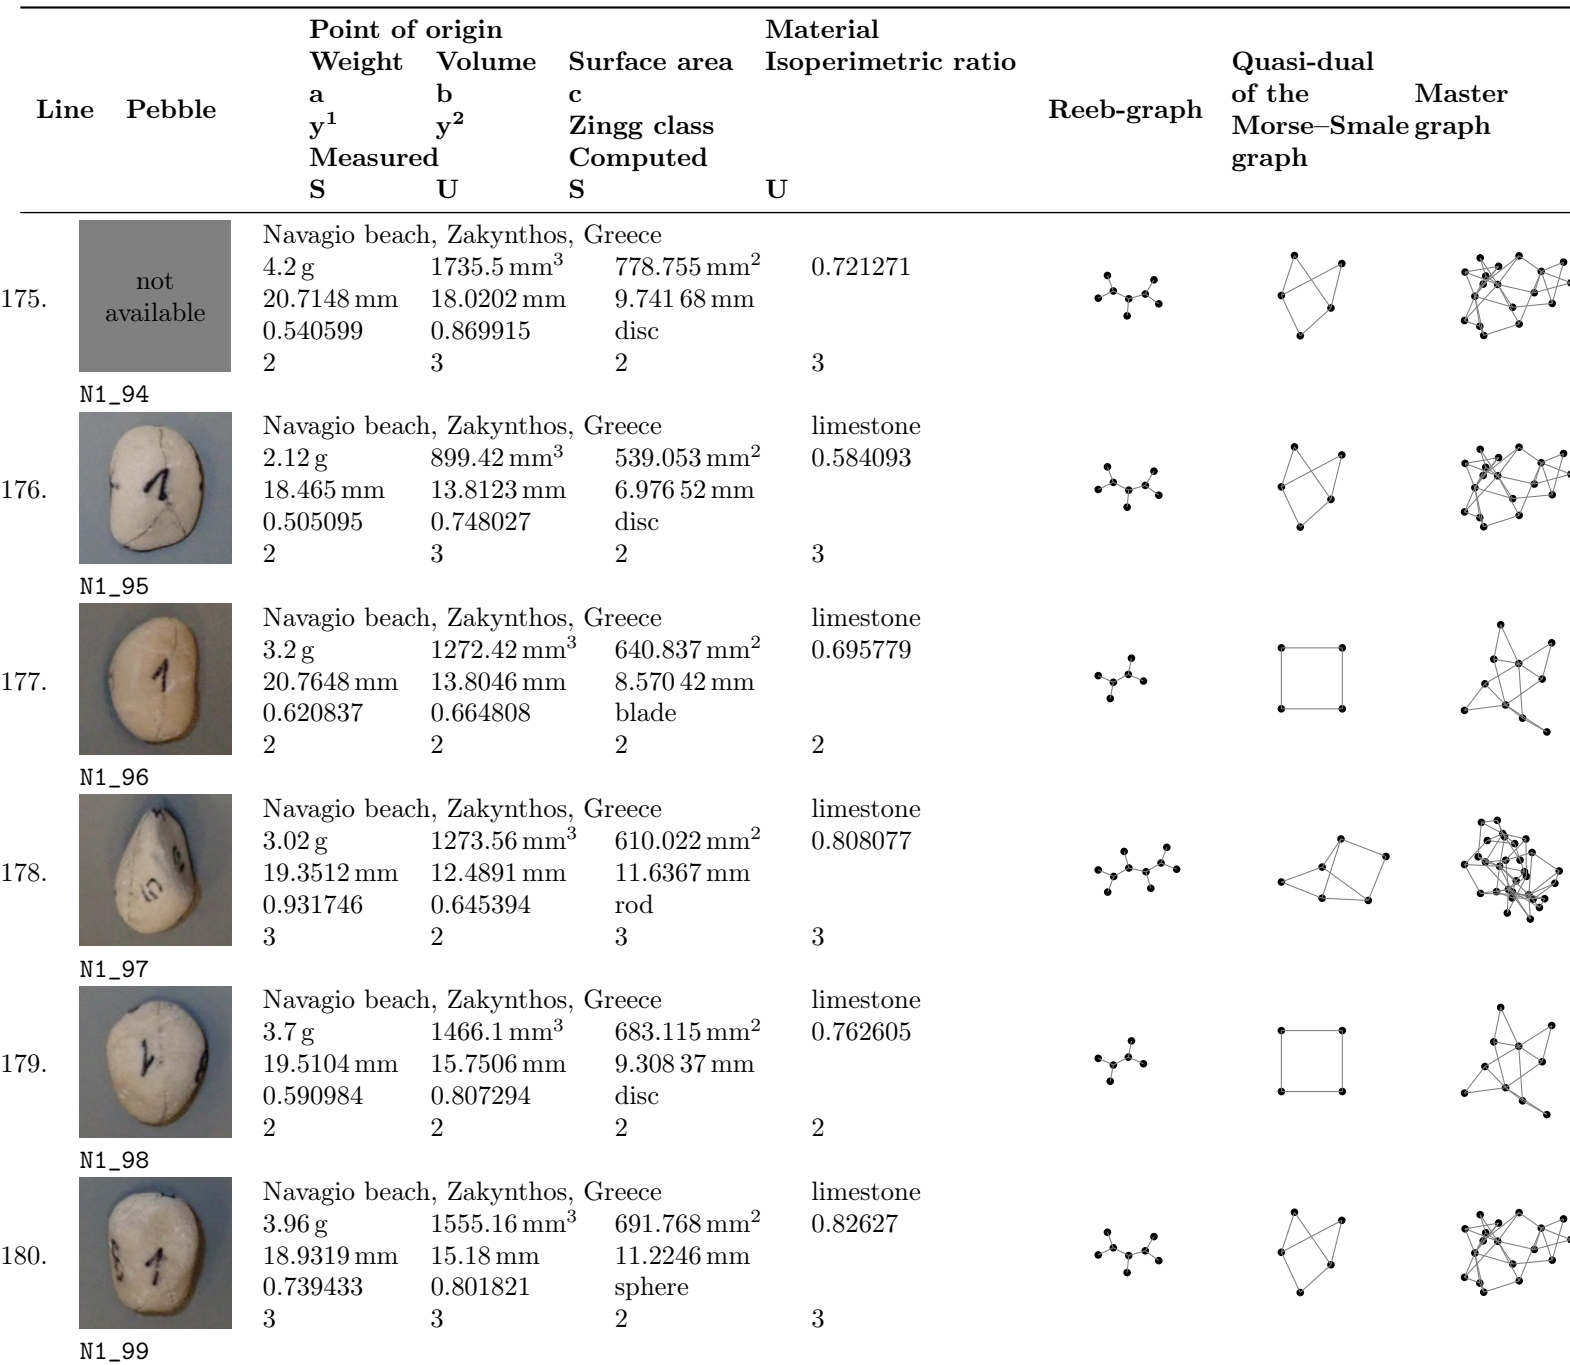 | 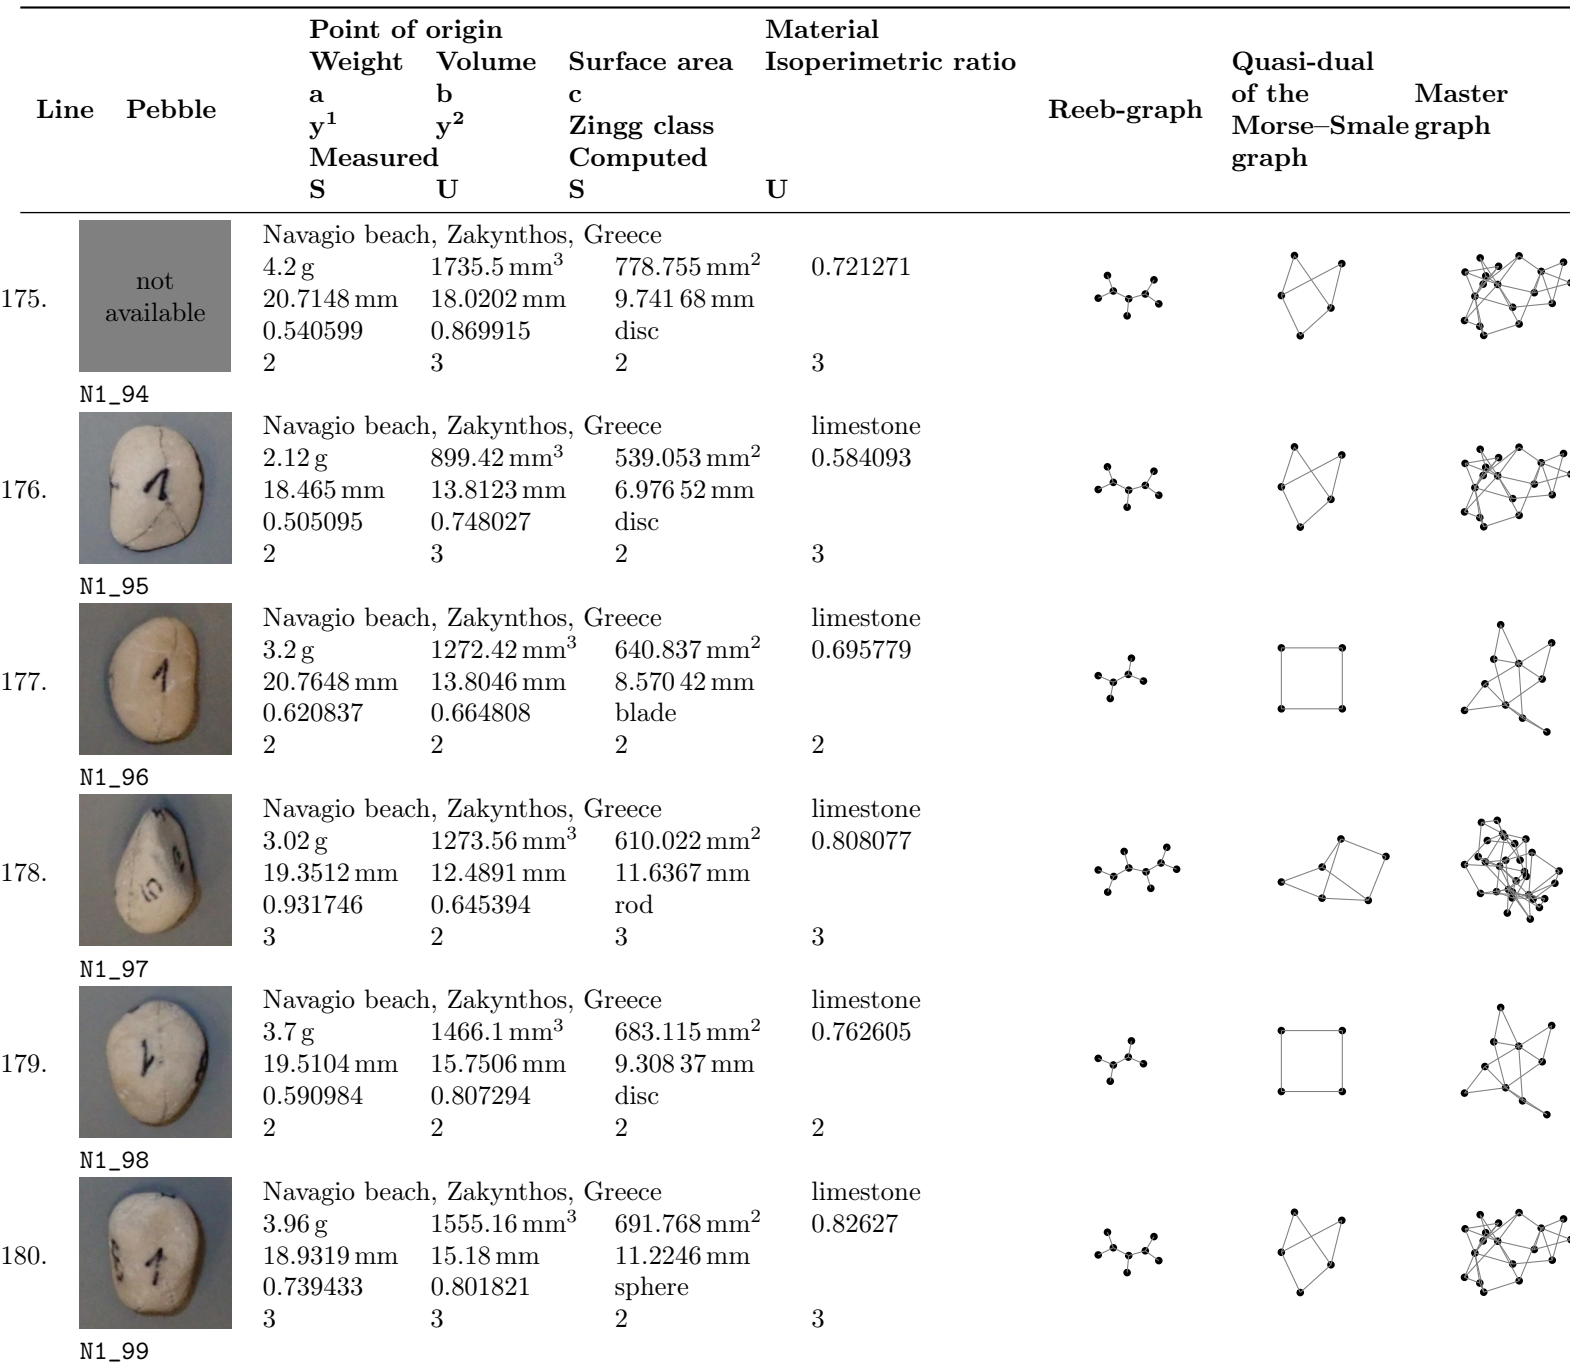 |
|      |                                                                                     | 3.96 g                               | 1555.16 mm <sup>3</sup>  | 691.768 mm <sup>2</sup>                           |                                      |                                                                                       |                                                                                       |                                                                                       |
|      |                                                                                     | 18.9319 mm                           | 15.18 mm                 | 11.2246 mm                                        |                                      |                                                                                       |                                                                                       |                                                                                       |
|      |                                                                                     | 0.739433                             | 0.801821                 | sphere                                            |                                      |                                                                                       |                                                                                       |                                                                                       |
|      |                                                                                     | 3                                    | 3                        | 2                                                 |                                      |                                                                                       |                                                                                       |                                                                                       |
|      | N1_99                                                                               |                                      |                          |                                                   |                                      |                                                                                       |                                                                                       |                                                                                       |

| Line | Pebble                                                                              | Point of origin                                                                |                                                         |                                                      | Material                       | Reeb-graph                                                                            | Quasi-dual<br>of the<br>Morse–Smale<br>graph                                          | Master<br>graph                                                                       |
|------|-------------------------------------------------------------------------------------|--------------------------------------------------------------------------------|---------------------------------------------------------|------------------------------------------------------|--------------------------------|---------------------------------------------------------------------------------------|---------------------------------------------------------------------------------------|---------------------------------------------------------------------------------------|
|      |                                                                                     | Weight                                                                         | Volume                                                  | Surface area                                         |                                |                                                                                       |                                                                                       |                                                                                       |
|      |                                                                                     | a                                                                              | b                                                       | c                                                    |                                |                                                                                       |                                                                                       |                                                                                       |
|      |                                                                                     | y <sup>1</sup><br>Measured<br>S                                                | y <sup>2</sup><br>U                                     | Zingg class<br>Computed<br>S                         |                                |                                                                                       |                                                                                       |                                                                                       |
| 181. | 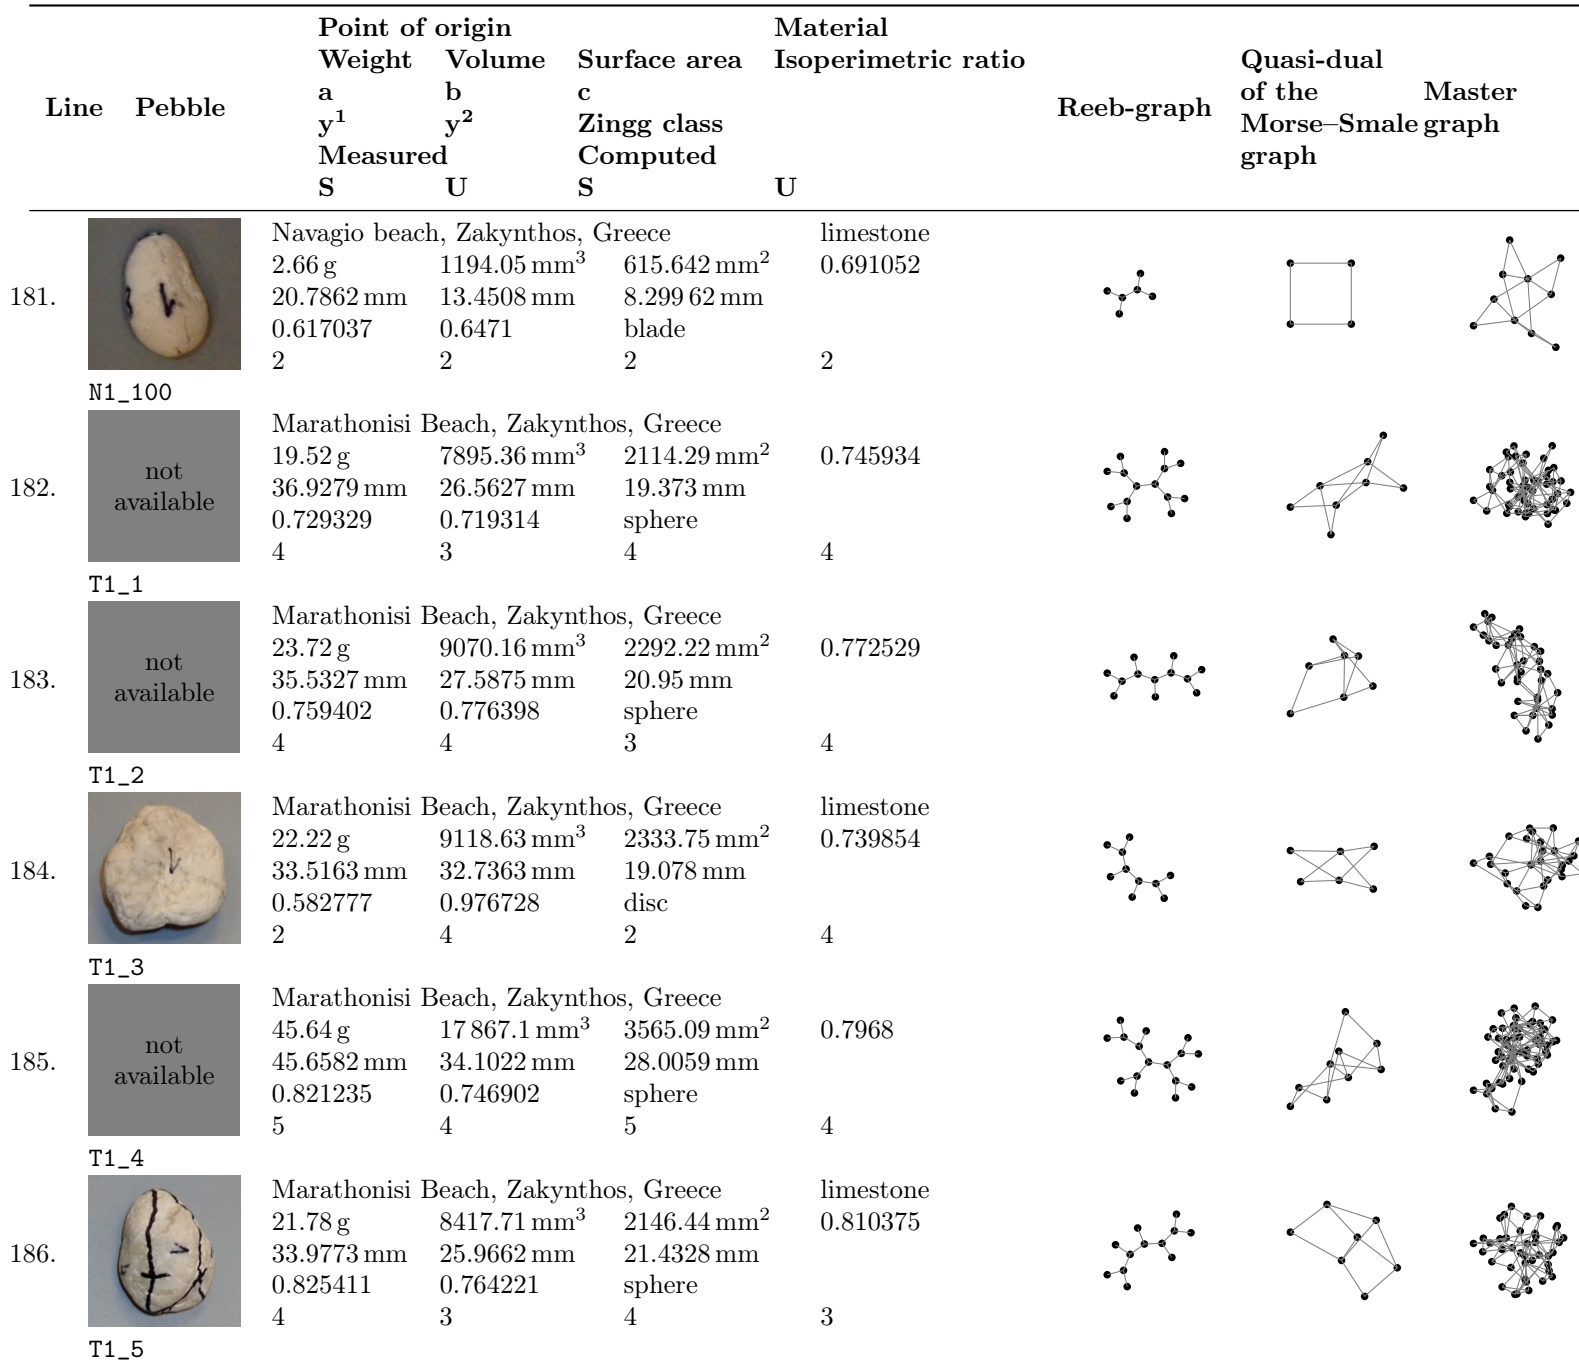   | Navagio beach, Zakynthos, Greece<br>2.66 g<br>20.7862 mm<br>0.617037<br>2      | 1194.05 mm <sup>3</sup><br>13.4508 mm<br>0.6471<br>2    | 615.642 mm <sup>2</sup><br>8.299 62 mm<br>blade<br>2 | limestone<br>0.691052<br><br>2 | 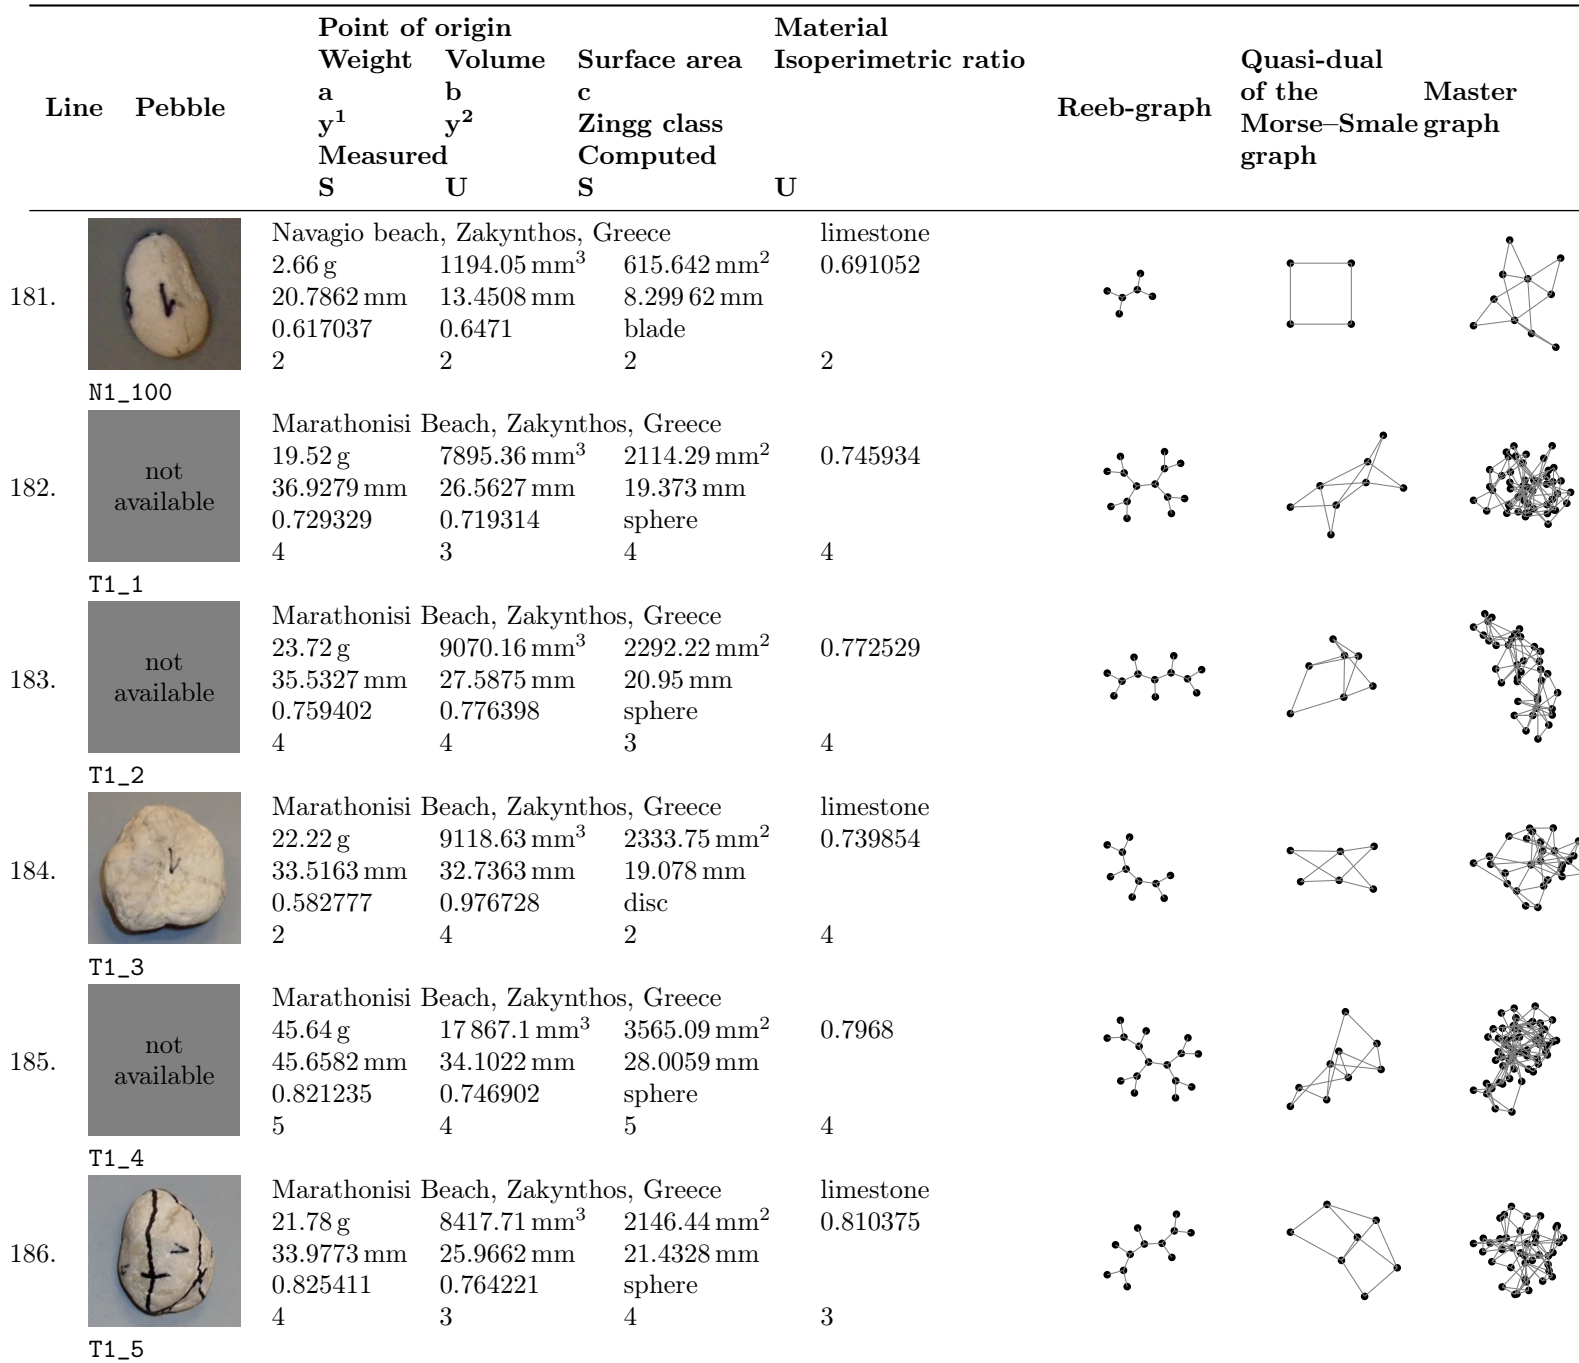   | 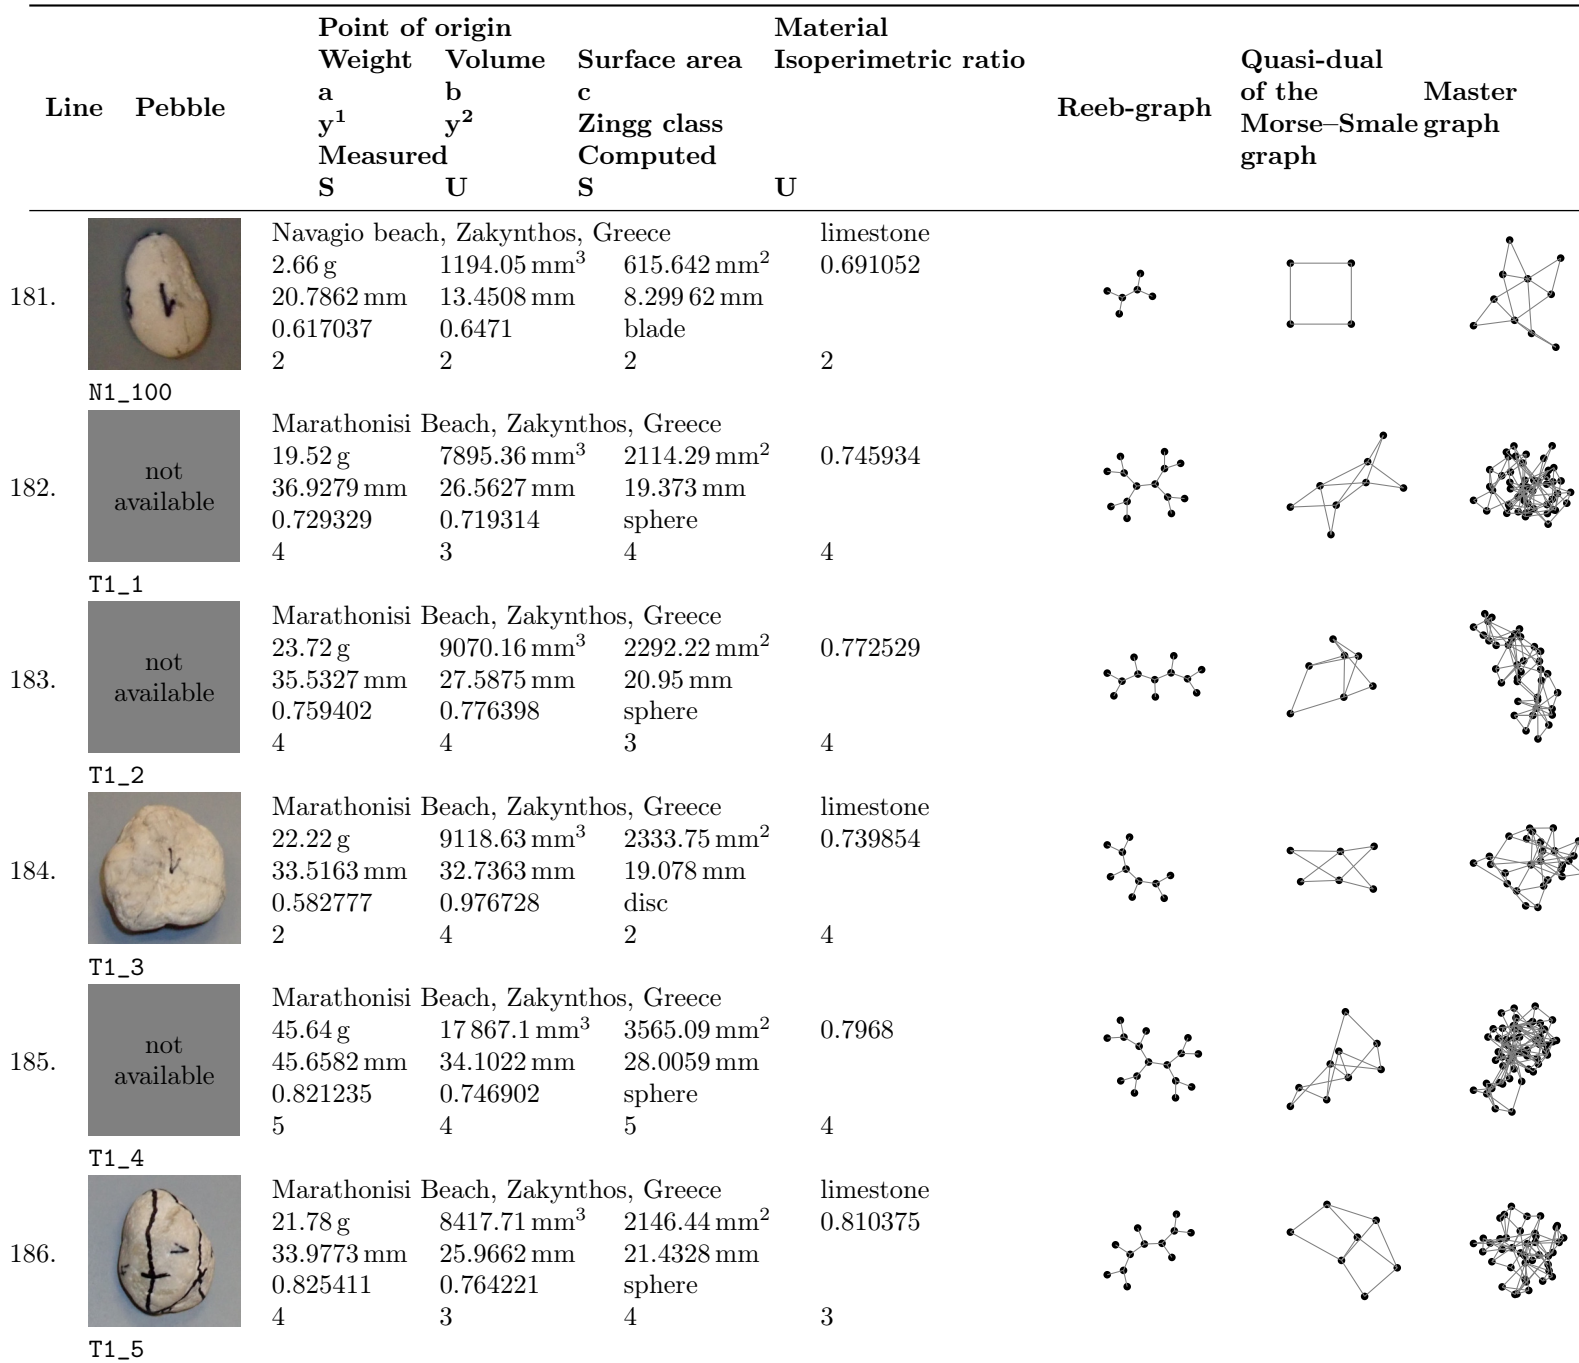   | 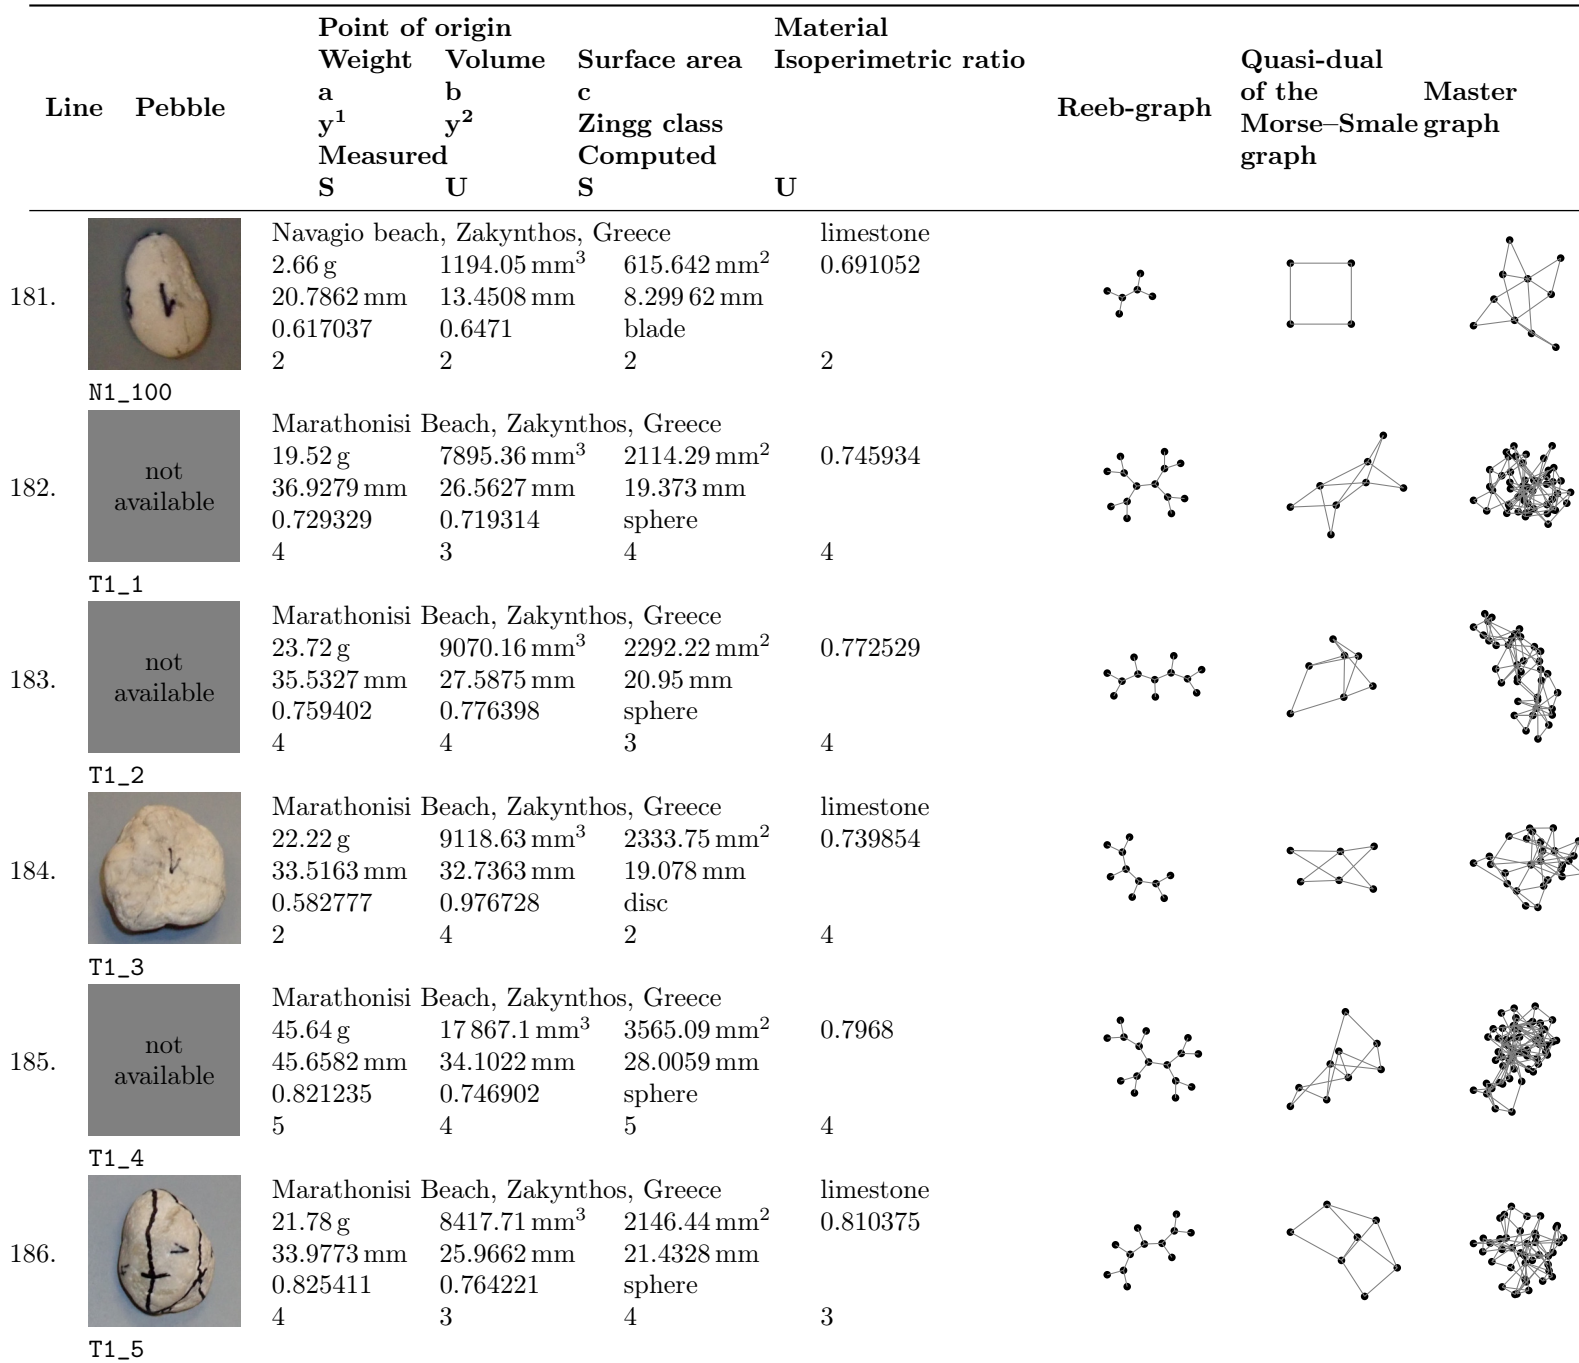   |
|      | N1_100                                                                              |                                                                                |                                                         |                                                      |                                |                                                                                       |                                                                                       |                                                                                       |
| 182. | 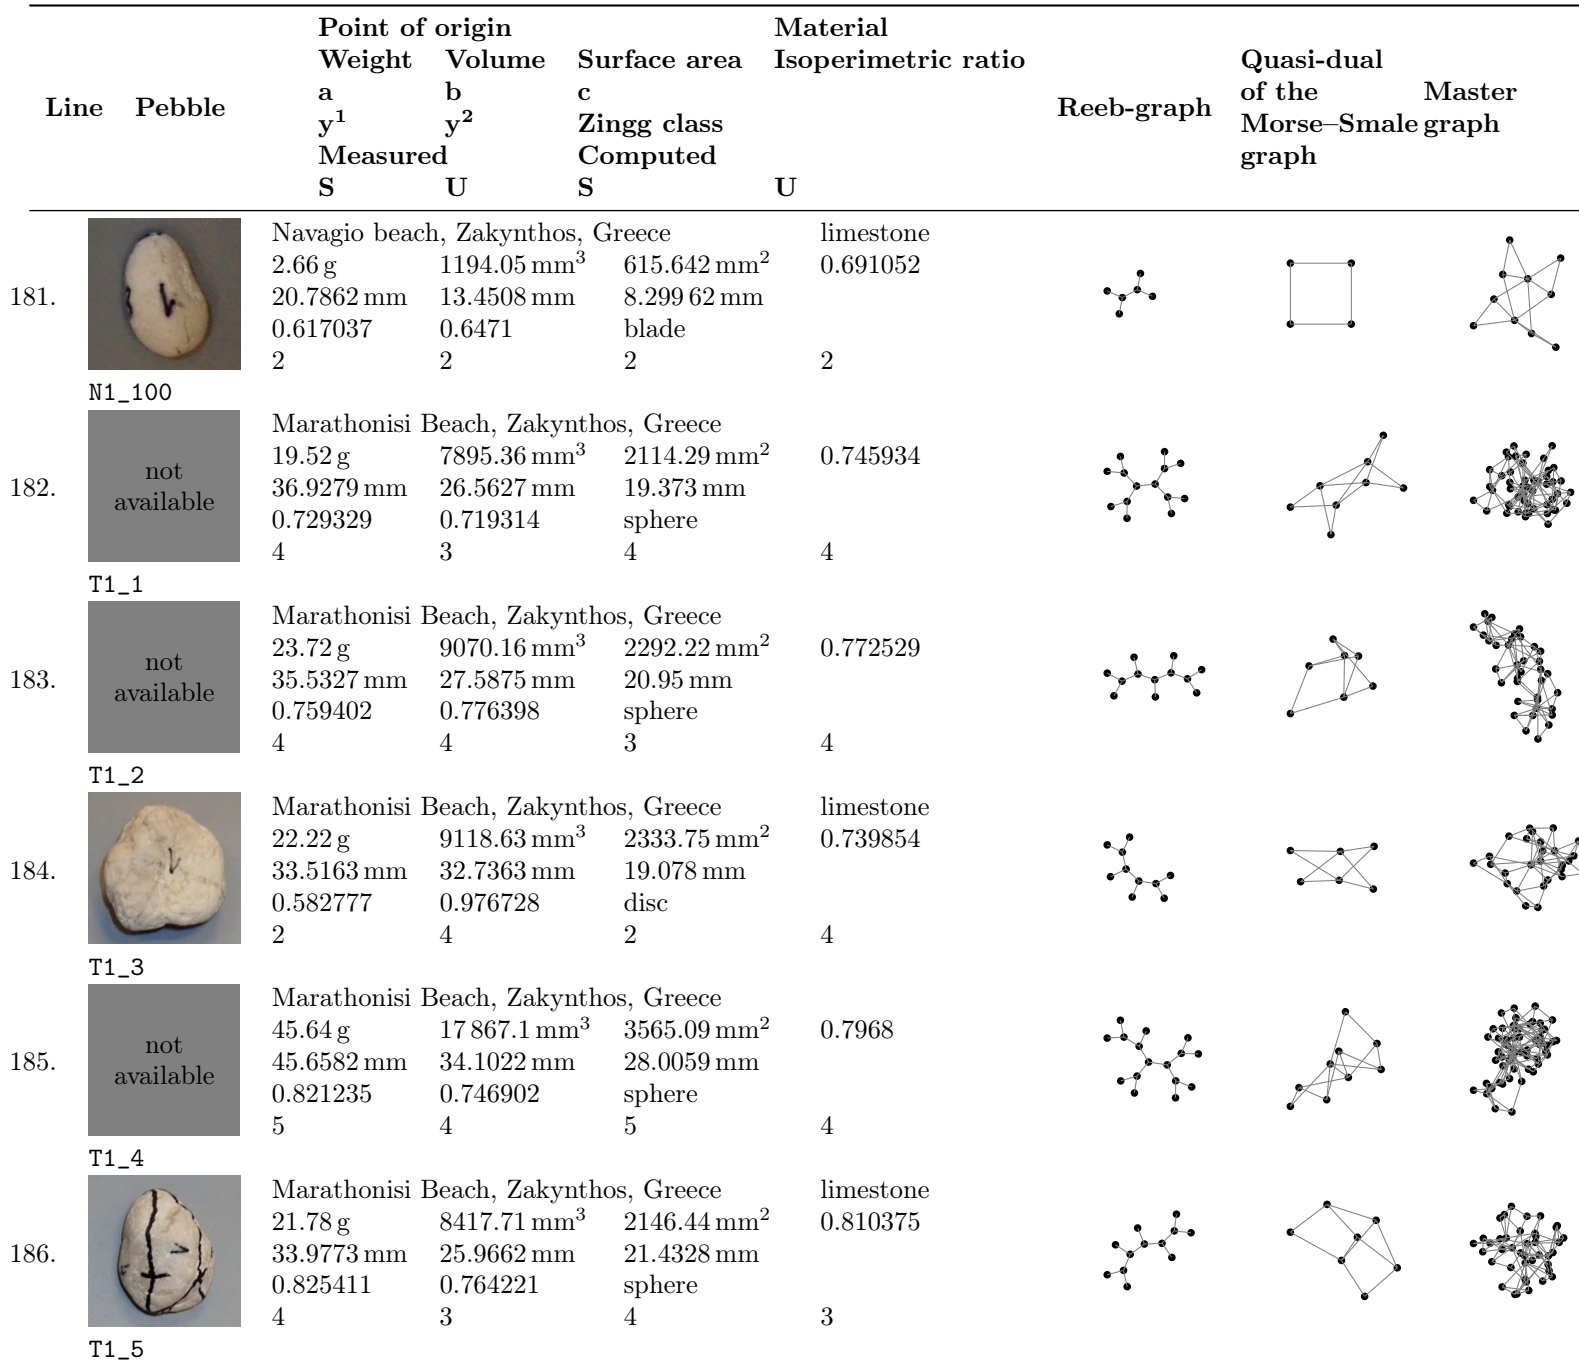   | Marathonisi Beach, Zakynthos, Greece<br>19.52 g<br>36.9279 mm<br>0.729329<br>4 | 7895.36 mm <sup>3</sup><br>26.5627 mm<br>0.719314<br>3  | 2114.29 mm <sup>2</sup><br>19.373 mm<br>sphere<br>4  | 0.745934<br><br>4              | 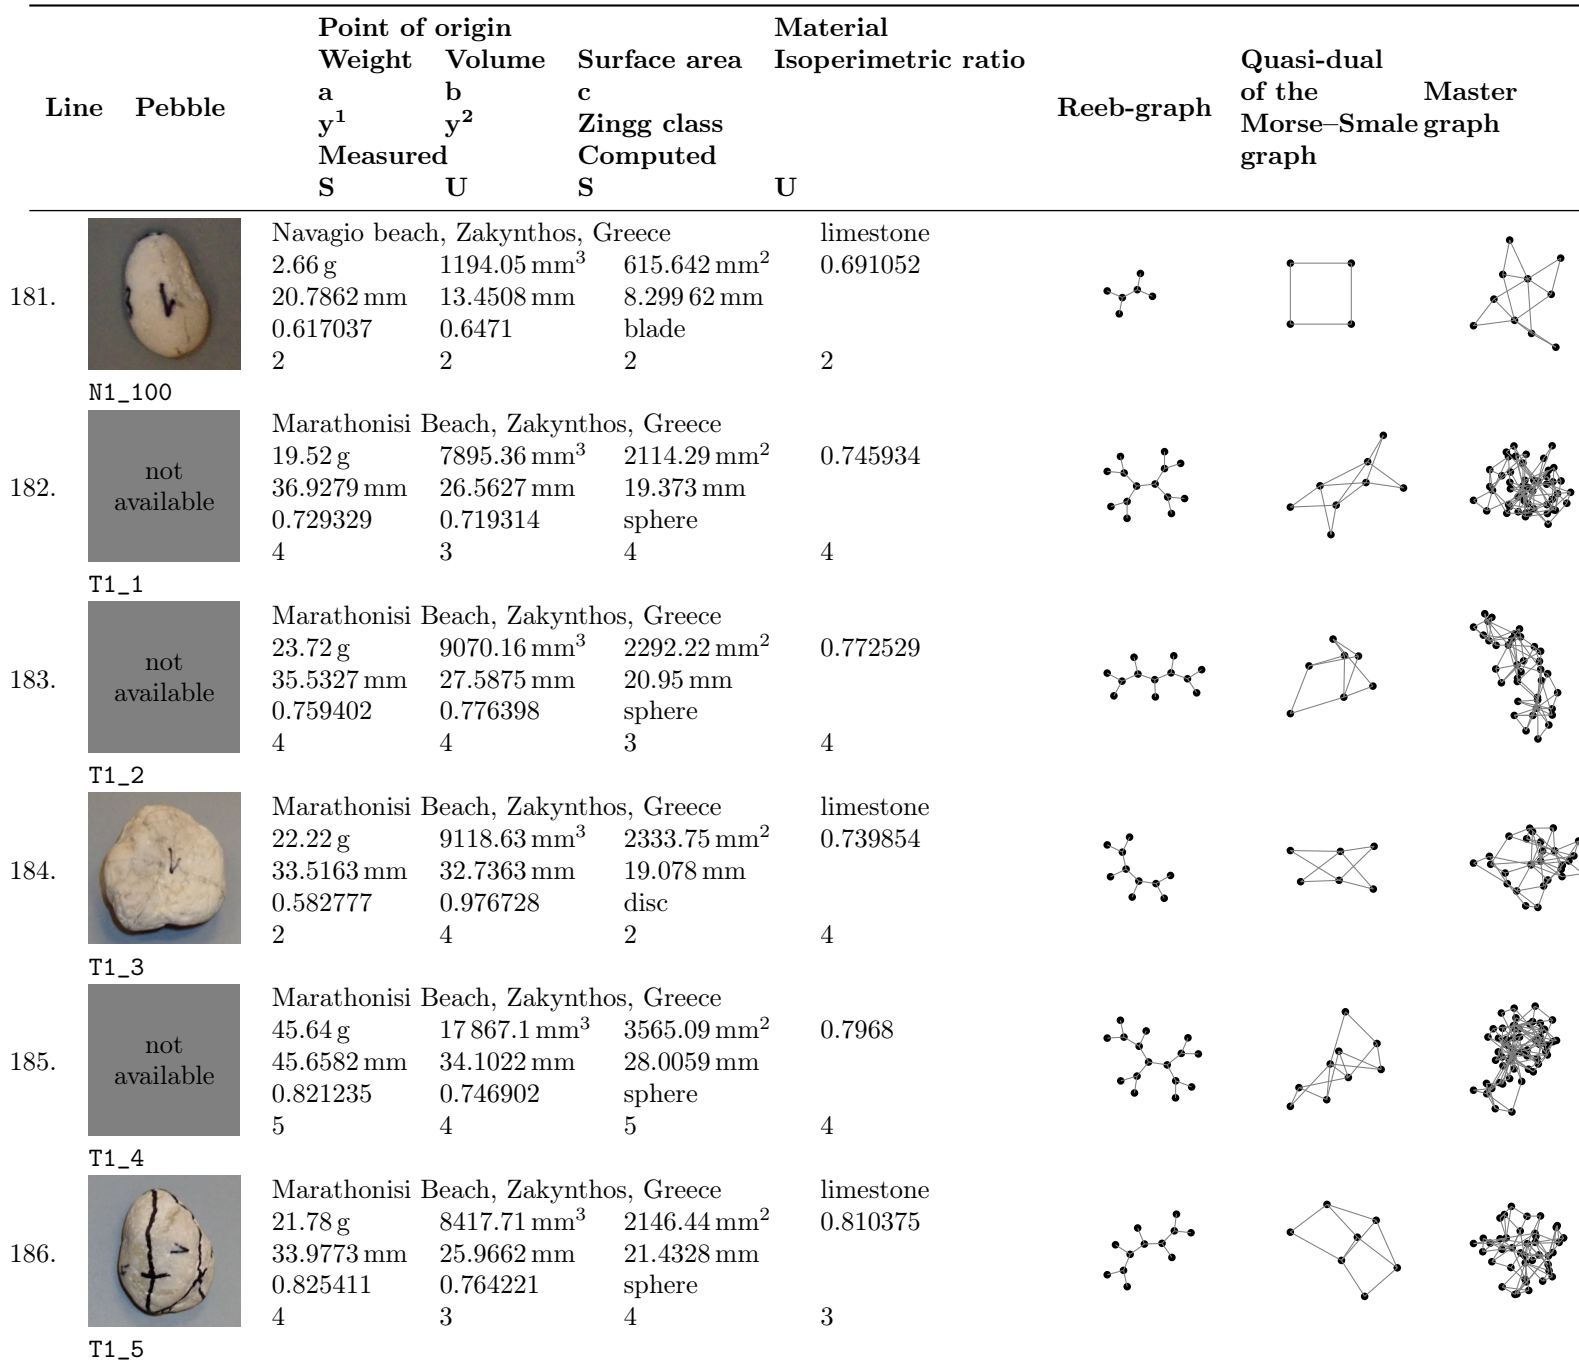   | 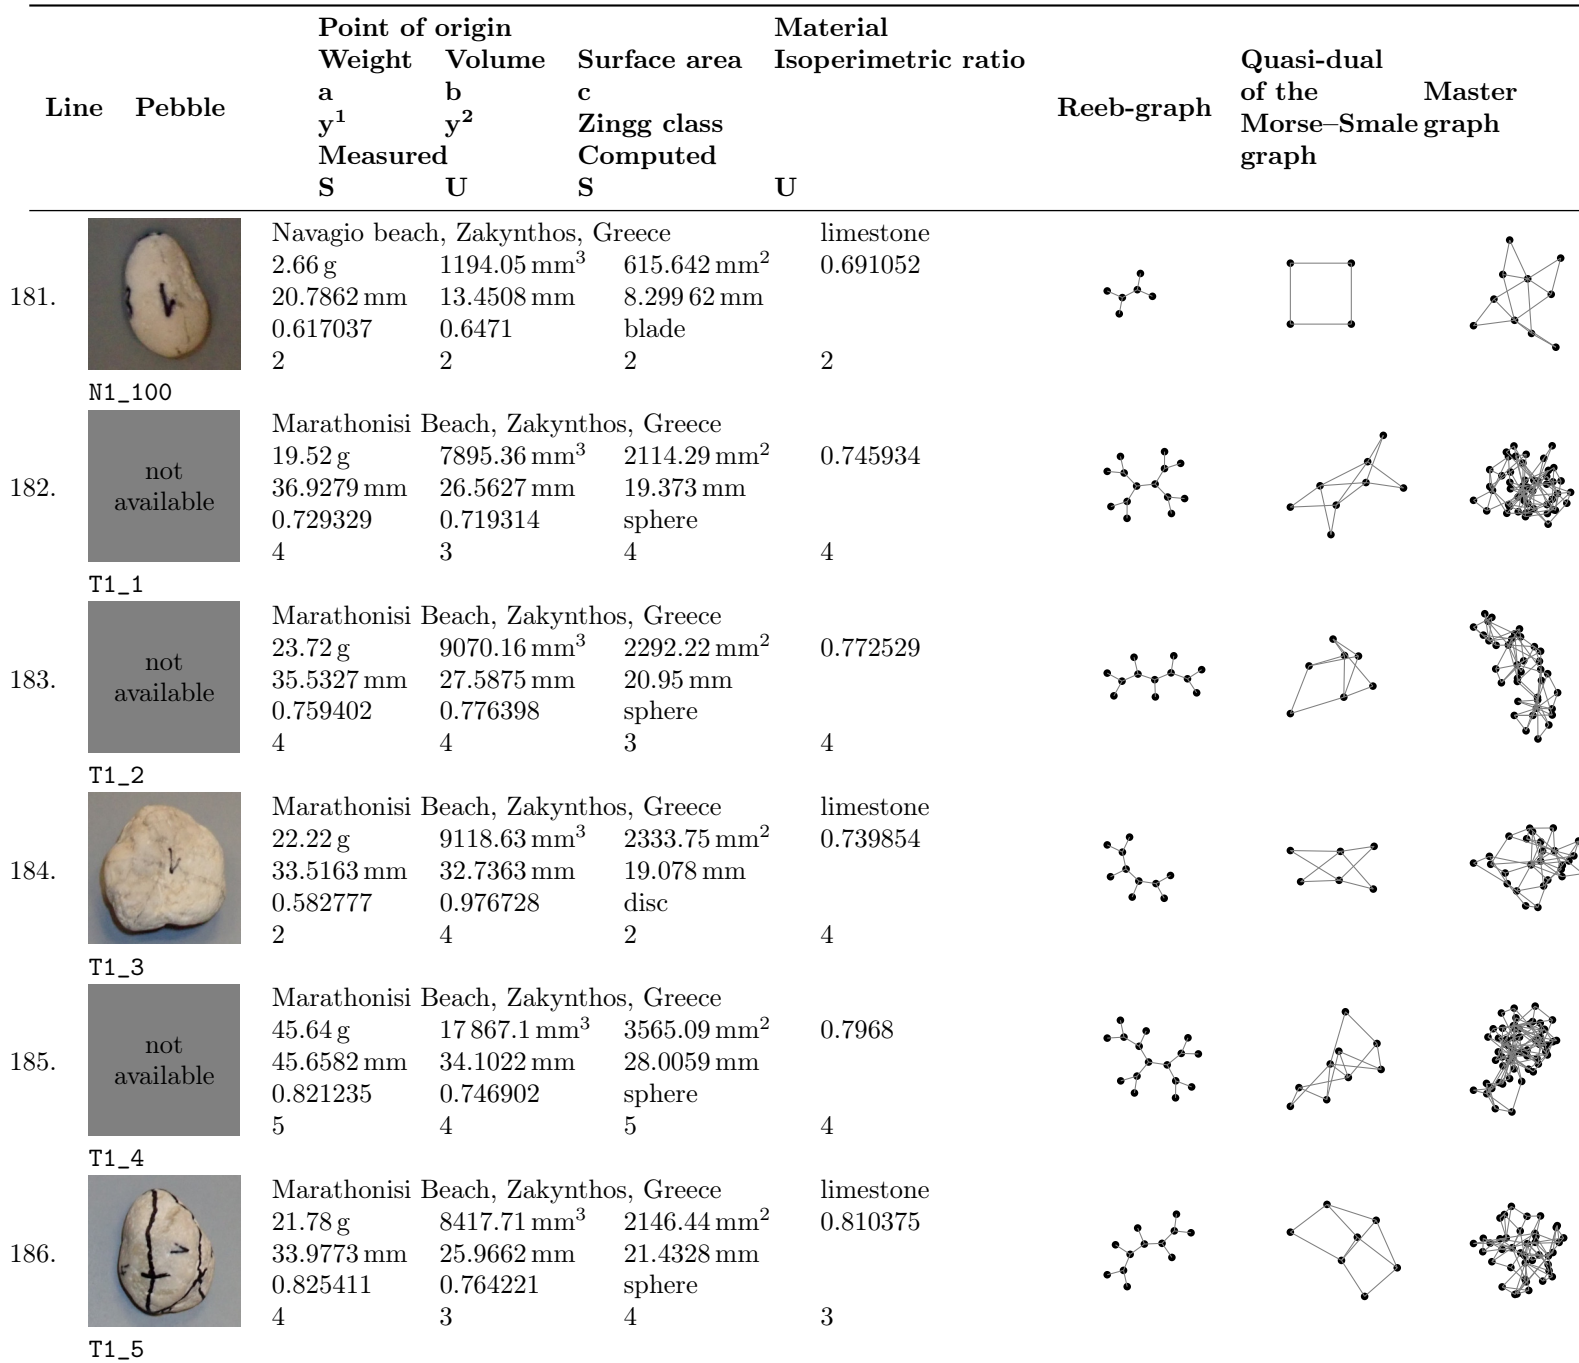   | 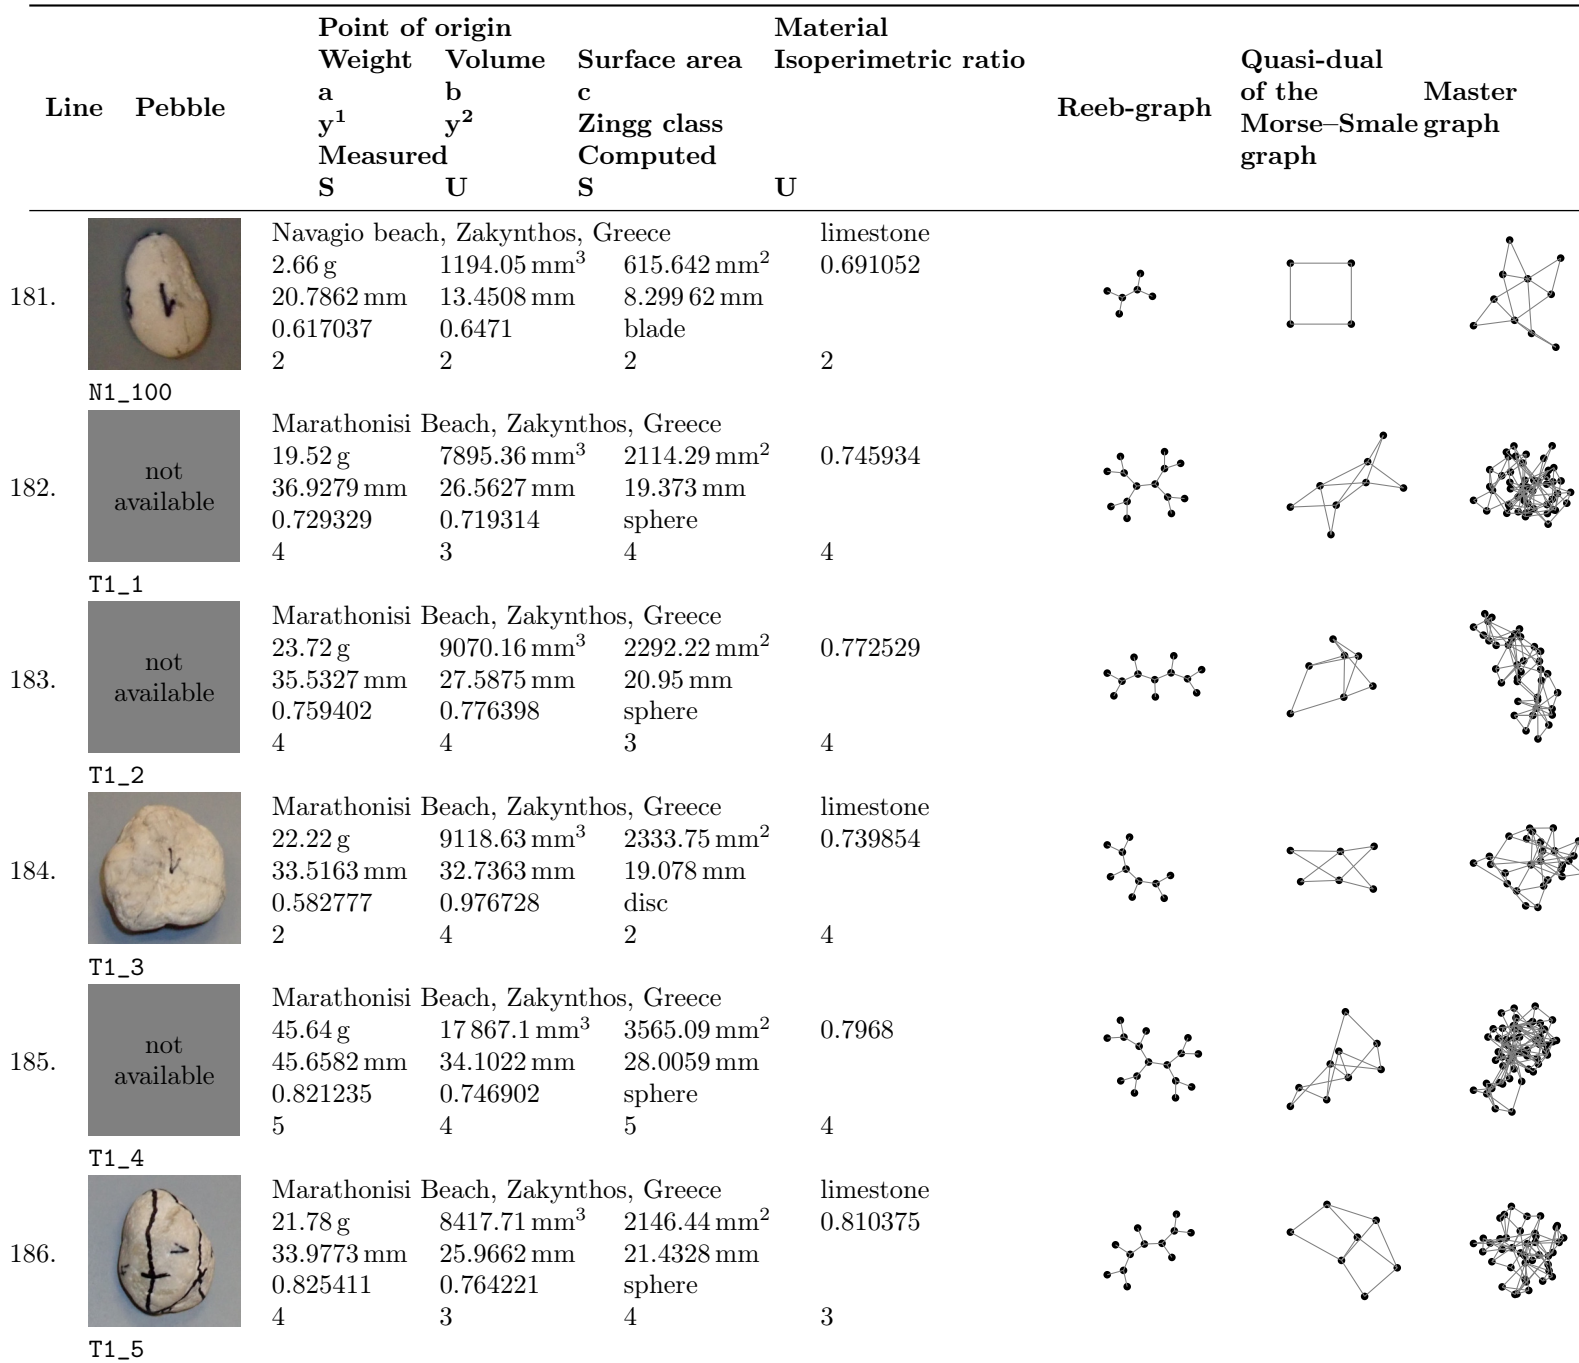   |
|      | T1_1                                                                                |                                                                                |                                                         |                                                      |                                |                                                                                       |                                                                                       |                                                                                       |
| 183. | 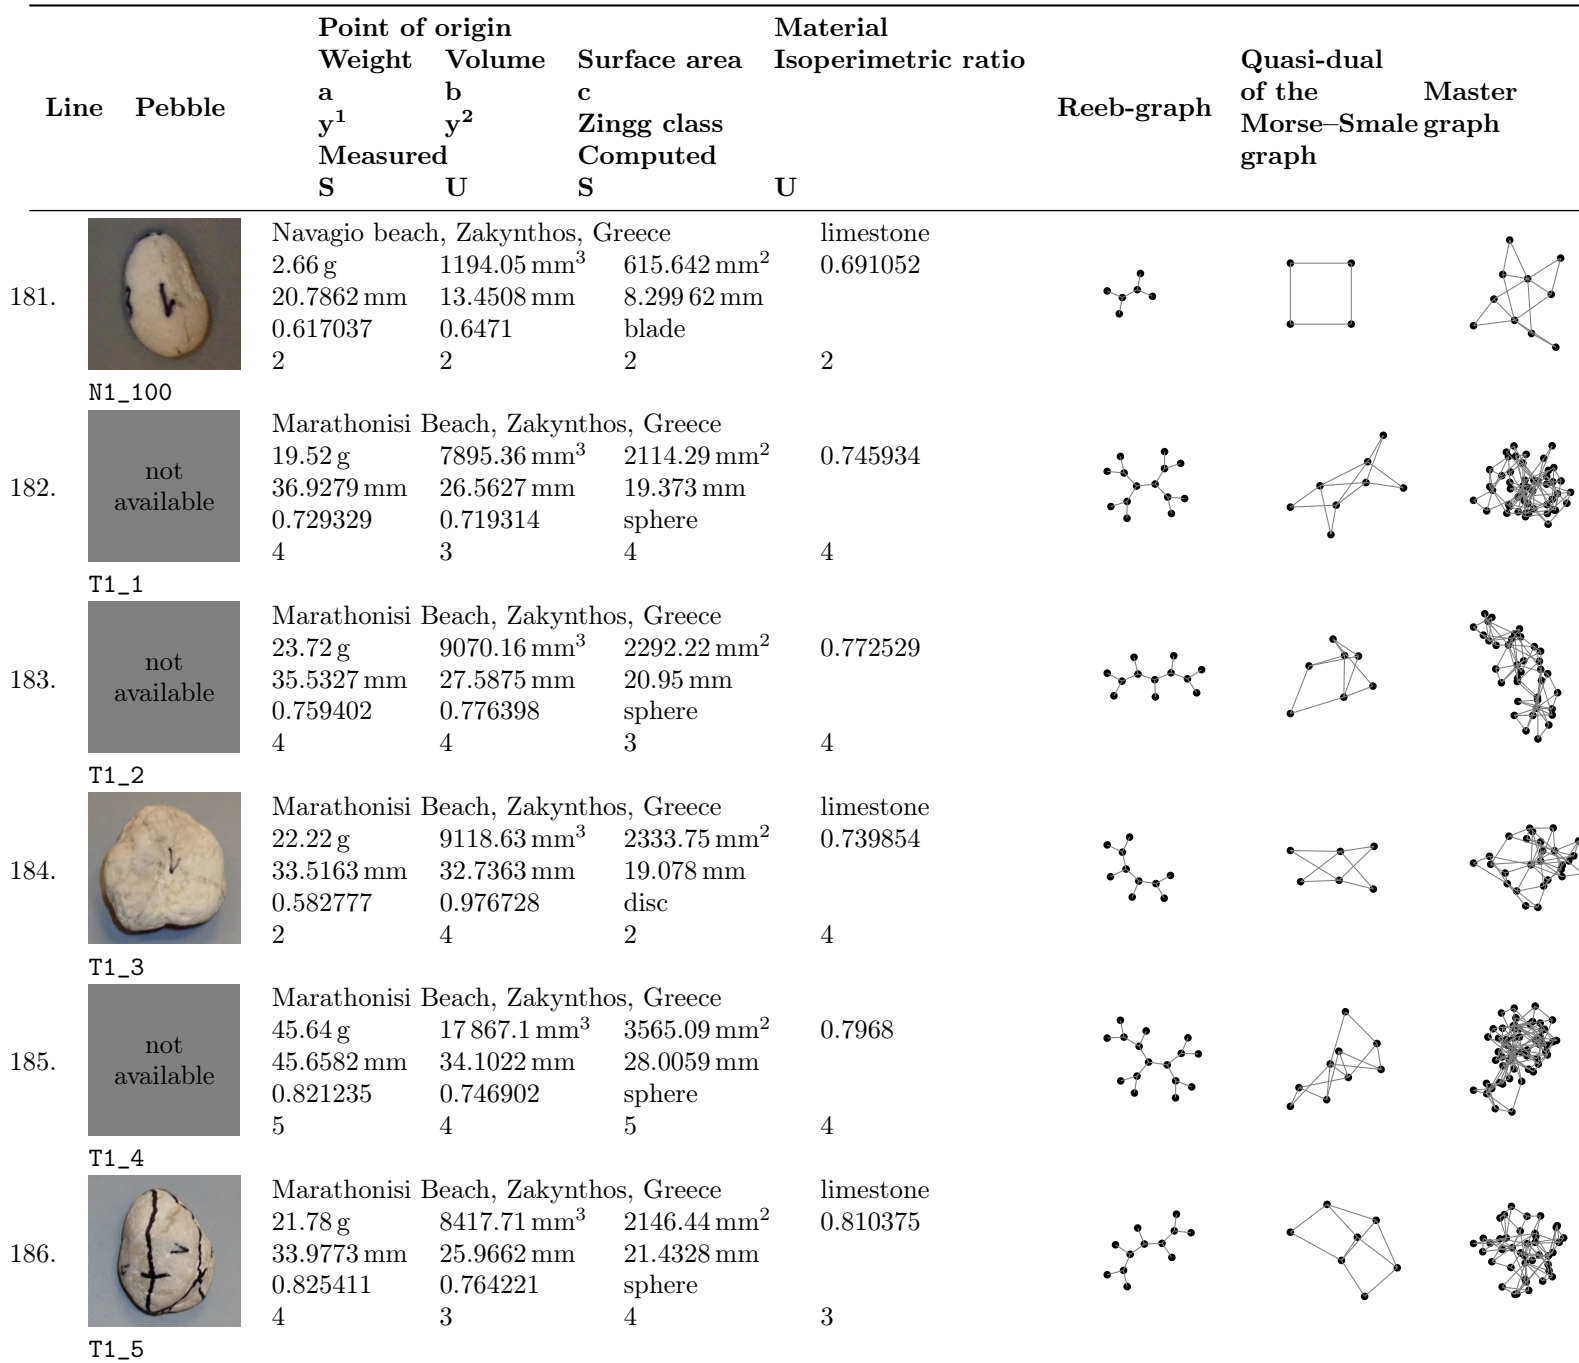   | Marathonisi Beach, Zakynthos, Greece<br>23.72 g<br>35.5327 mm<br>0.759402<br>4 | 9070.16 mm <sup>3</sup><br>27.5875 mm<br>0.776398<br>4  | 2292.22 mm <sup>2</sup><br>20.95 mm<br>sphere<br>3   | 0.772529<br><br>4              | 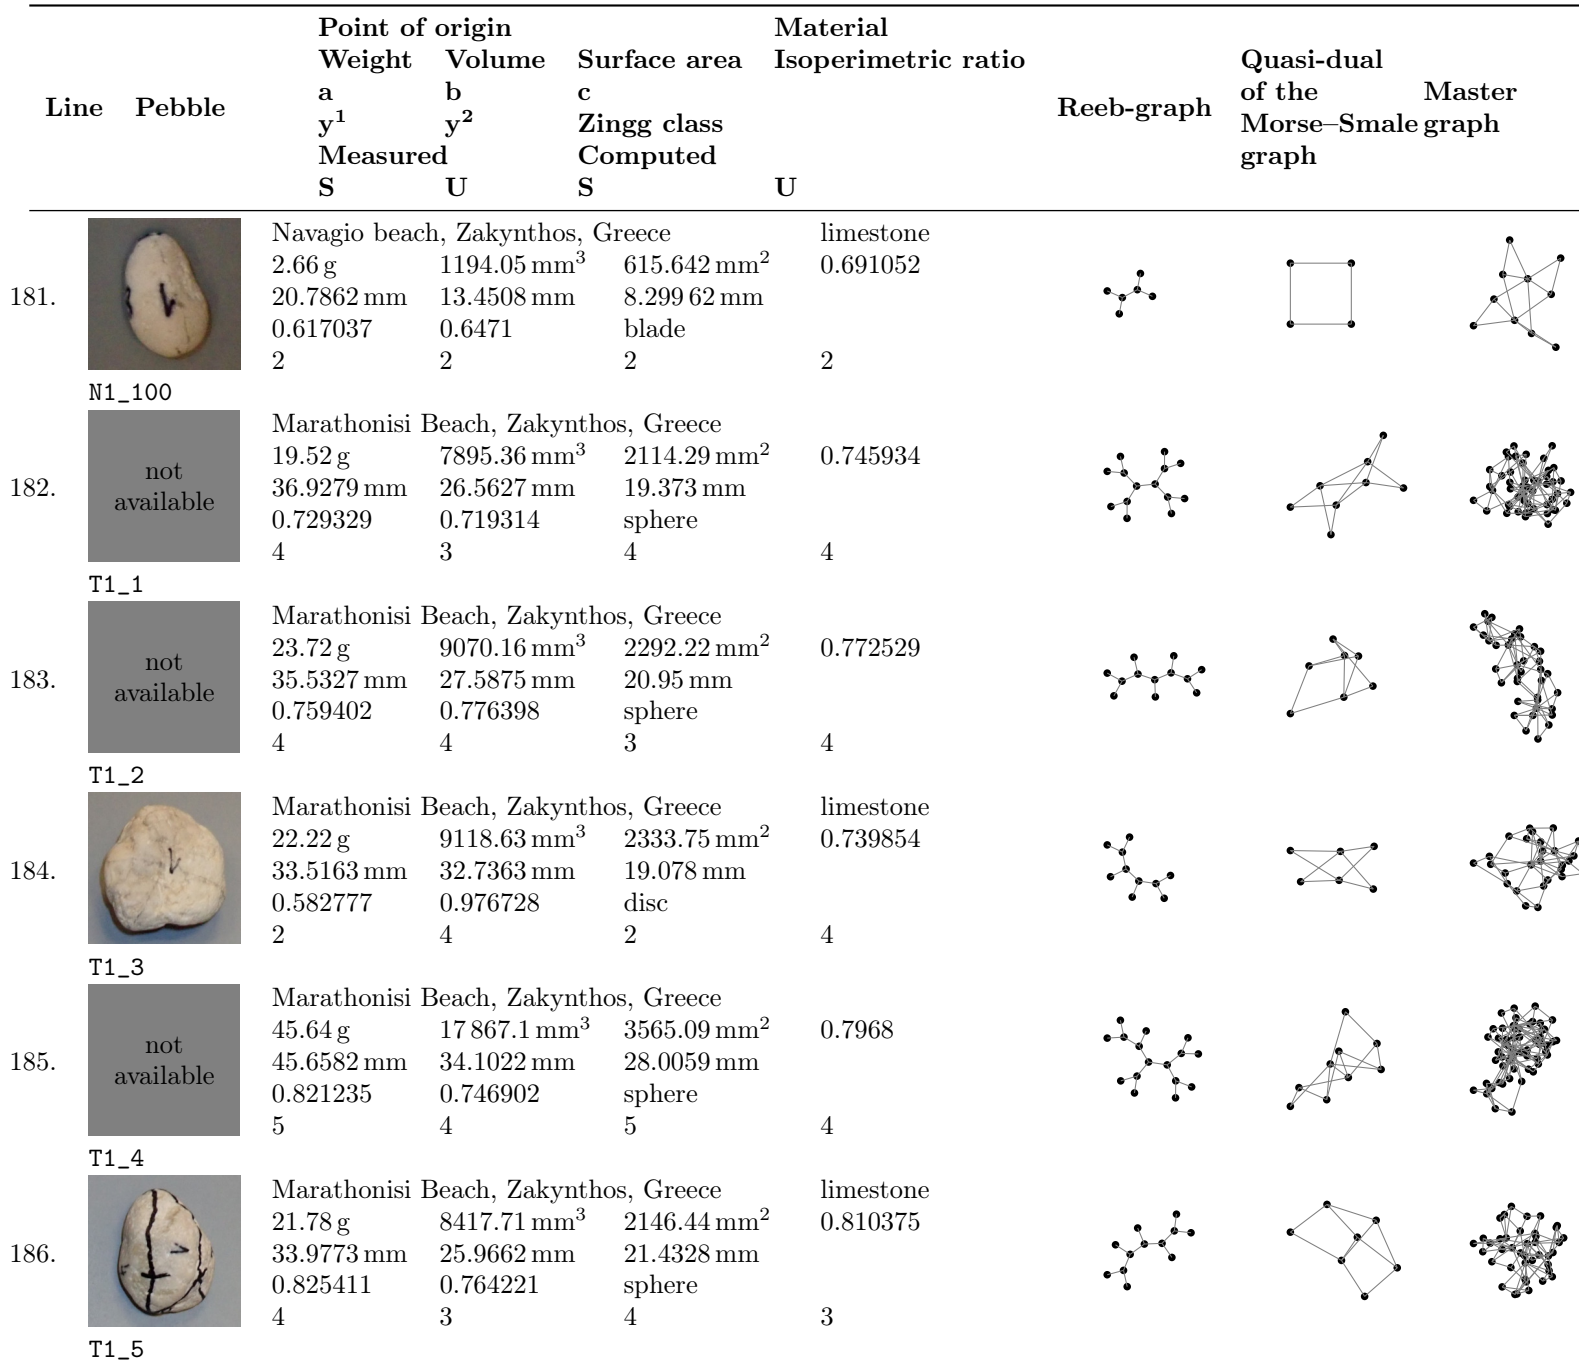   | 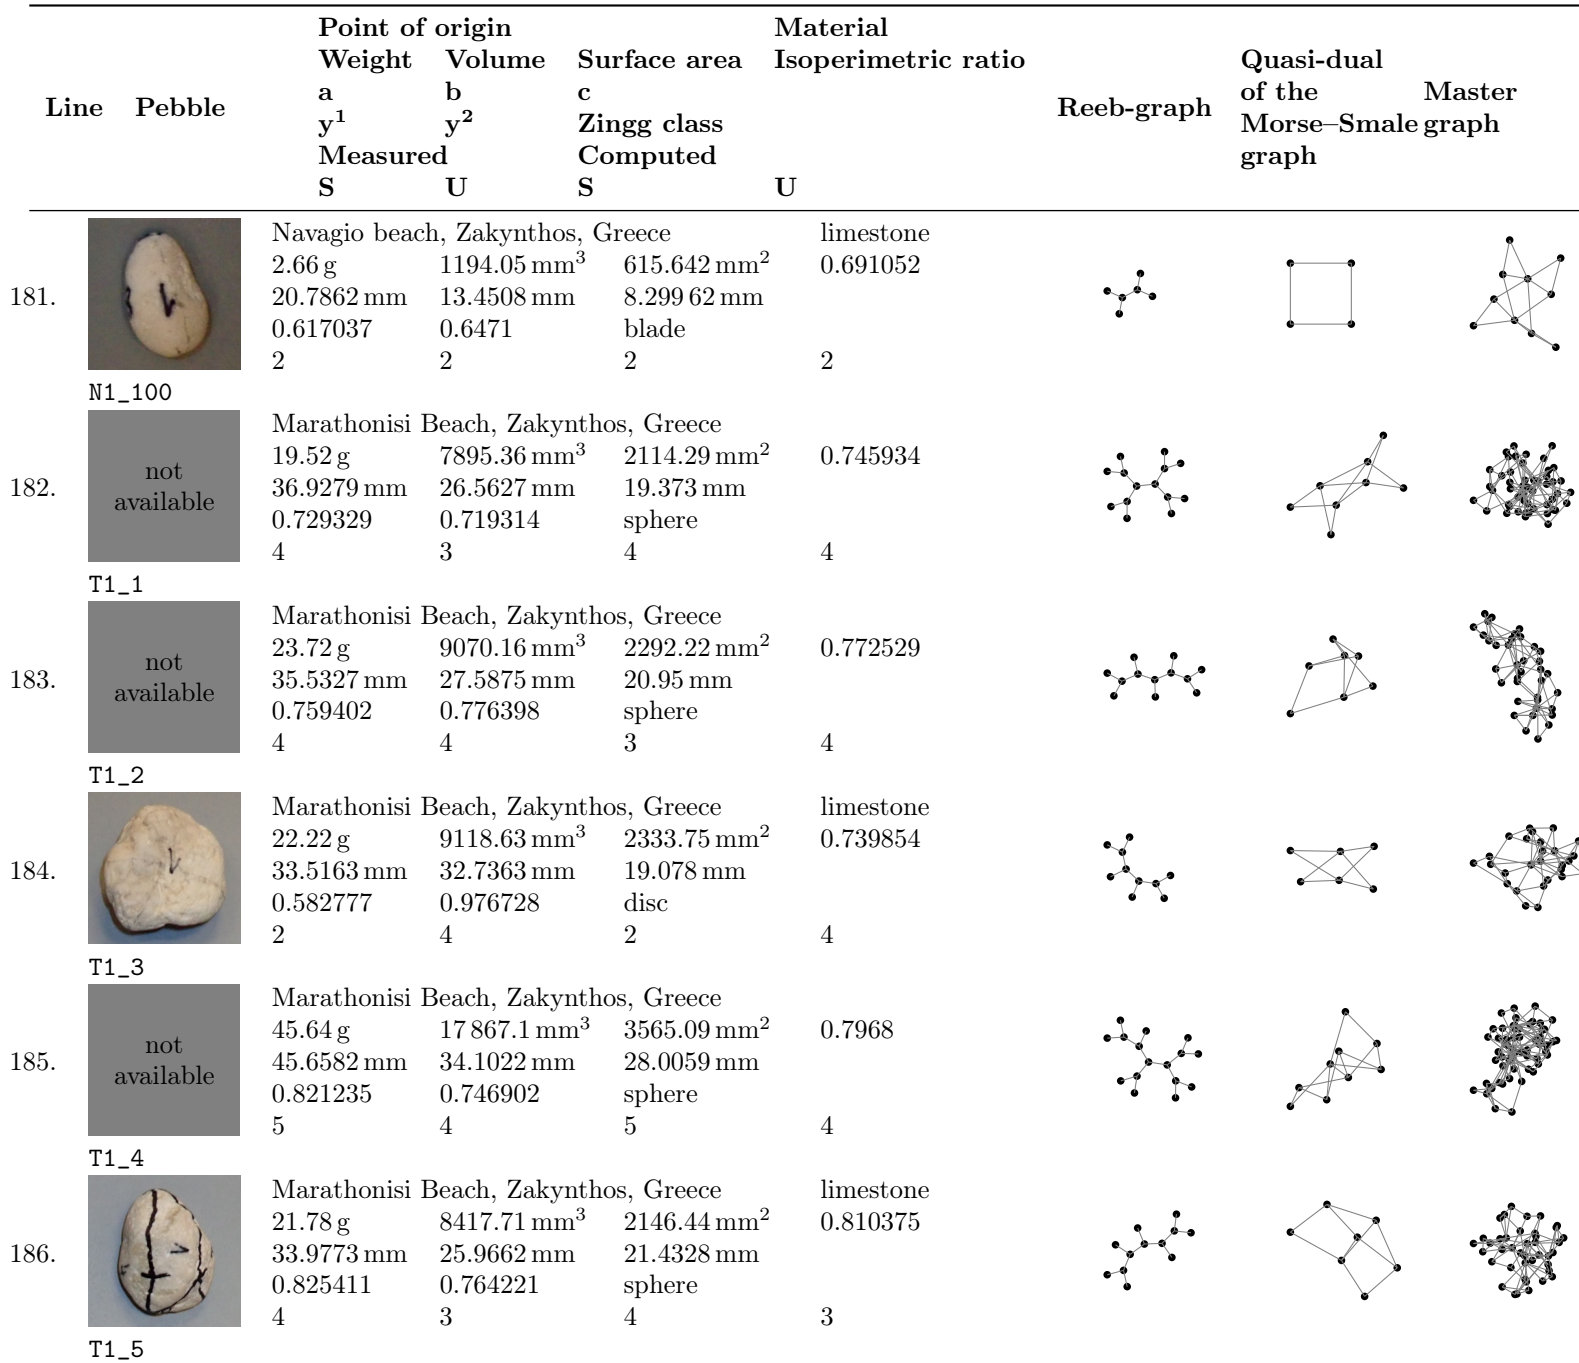   | 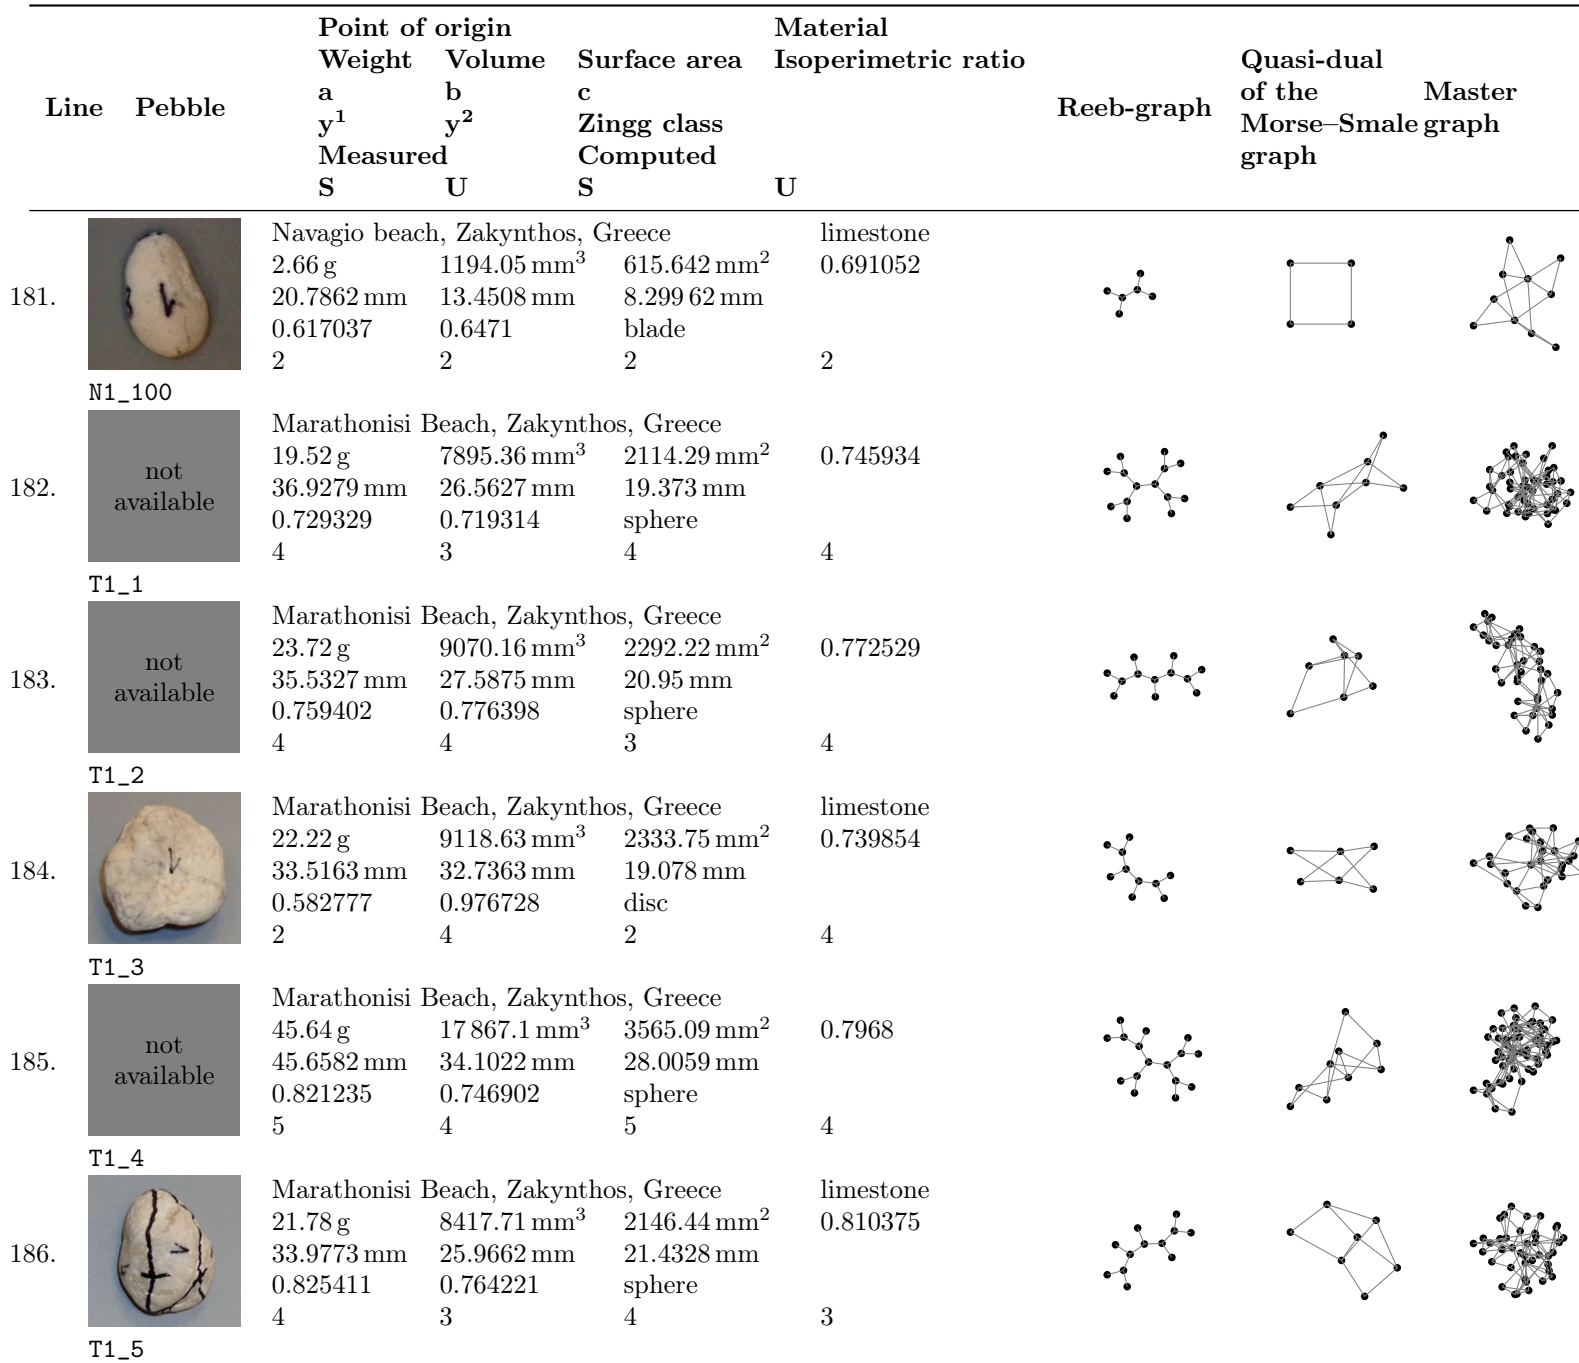   |
|      | T1_2                                                                                |                                                                                |                                                         |                                                      |                                |                                                                                       |                                                                                       |                                                                                       |
| 184. | 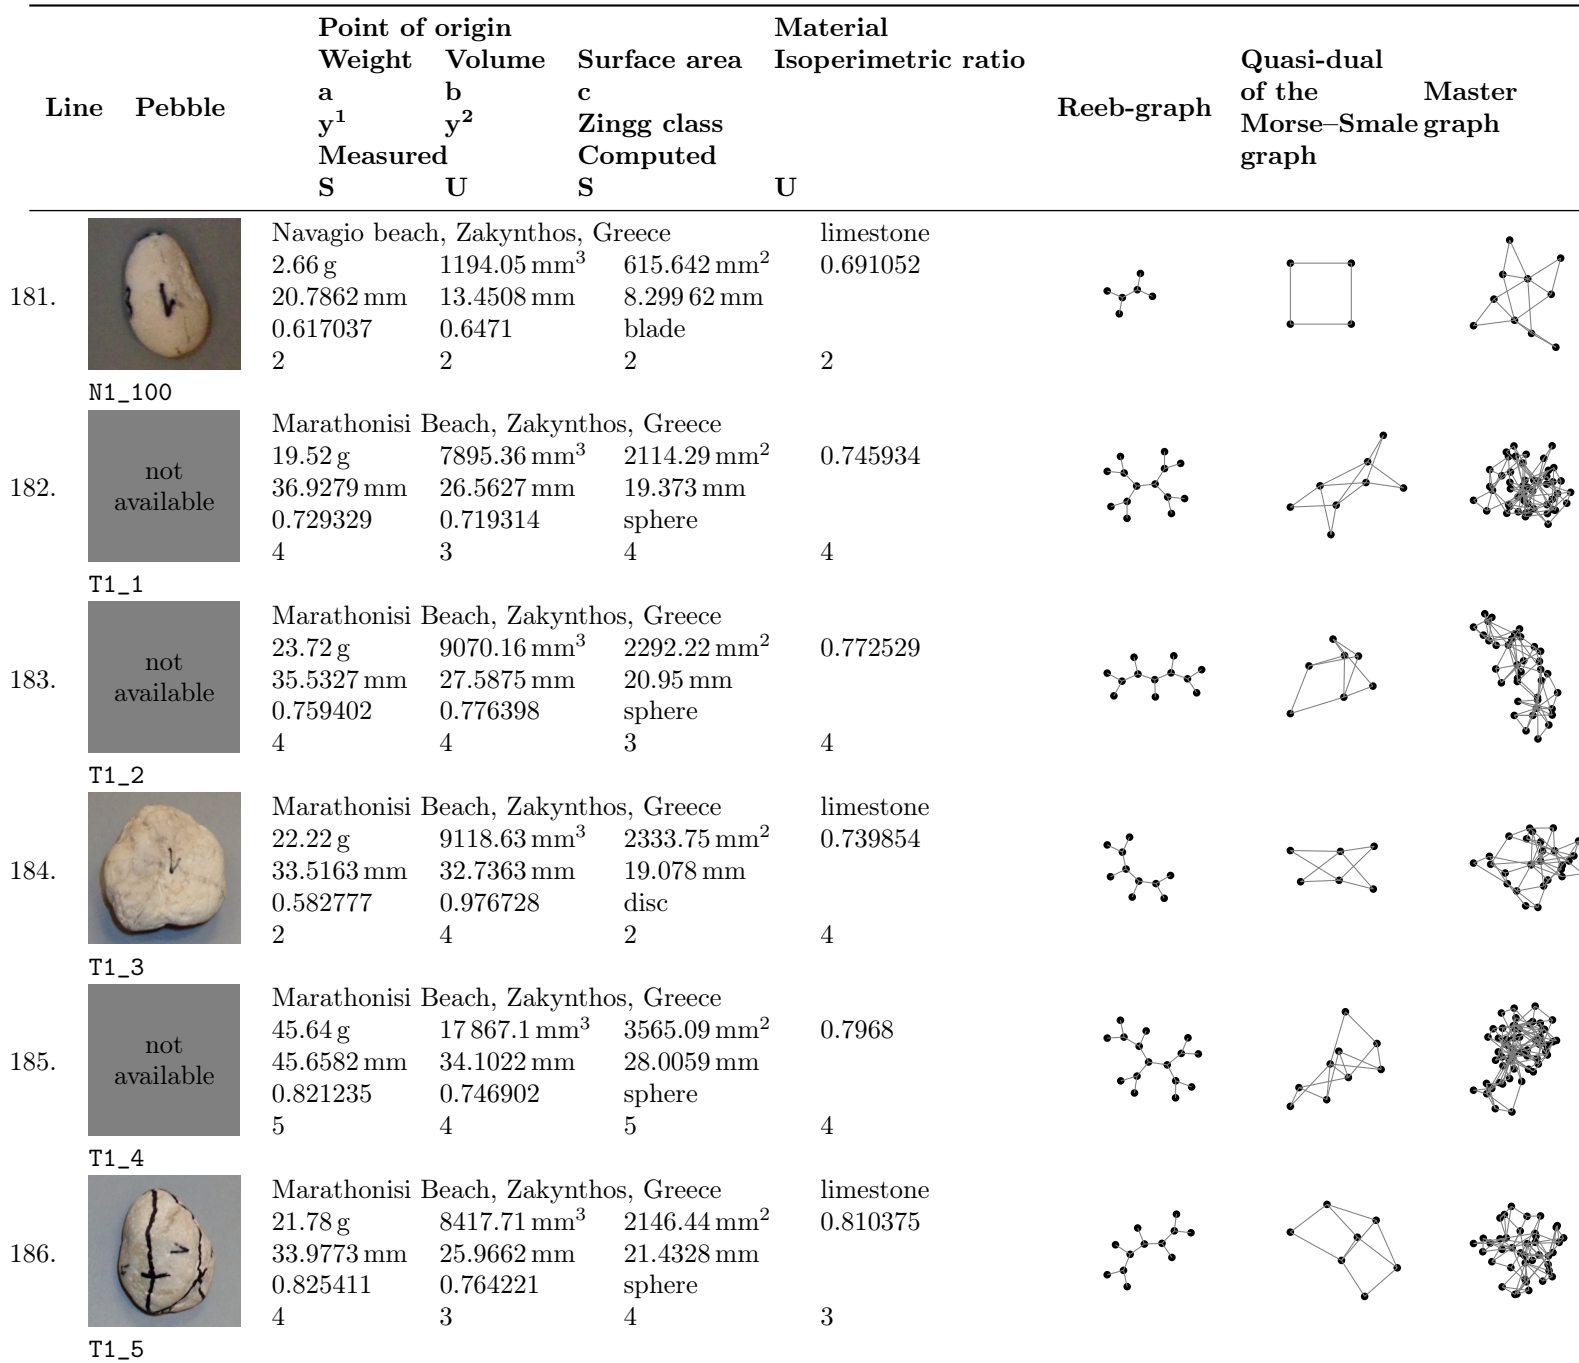  | Marathonisi Beach, Zakynthos, Greece<br>22.22 g<br>33.5163 mm<br>0.582777<br>2 | 9118.63 mm <sup>3</sup><br>32.7363 mm<br>0.976728<br>4  | 2333.75 mm <sup>2</sup><br>19.078 mm<br>disc<br>2    | limestone<br>0.739854<br><br>4 | 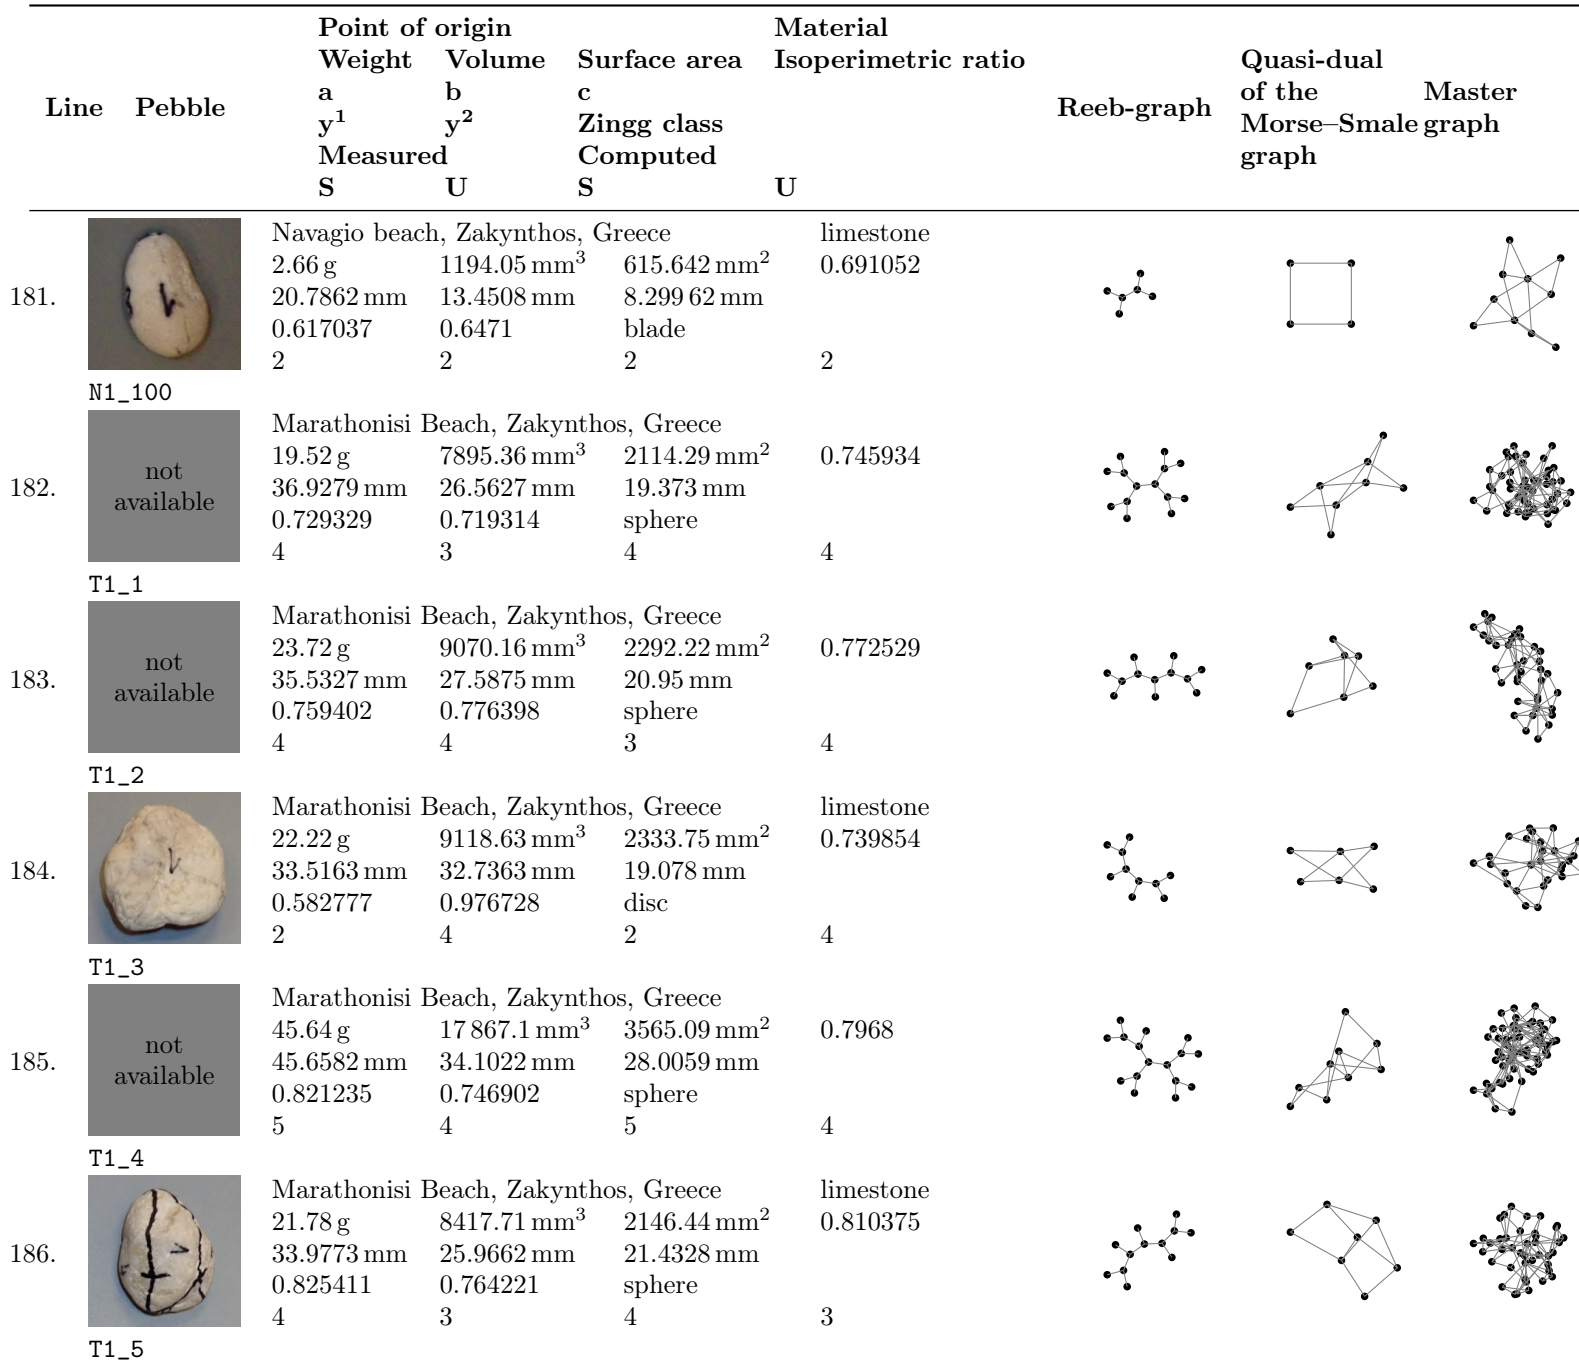  | 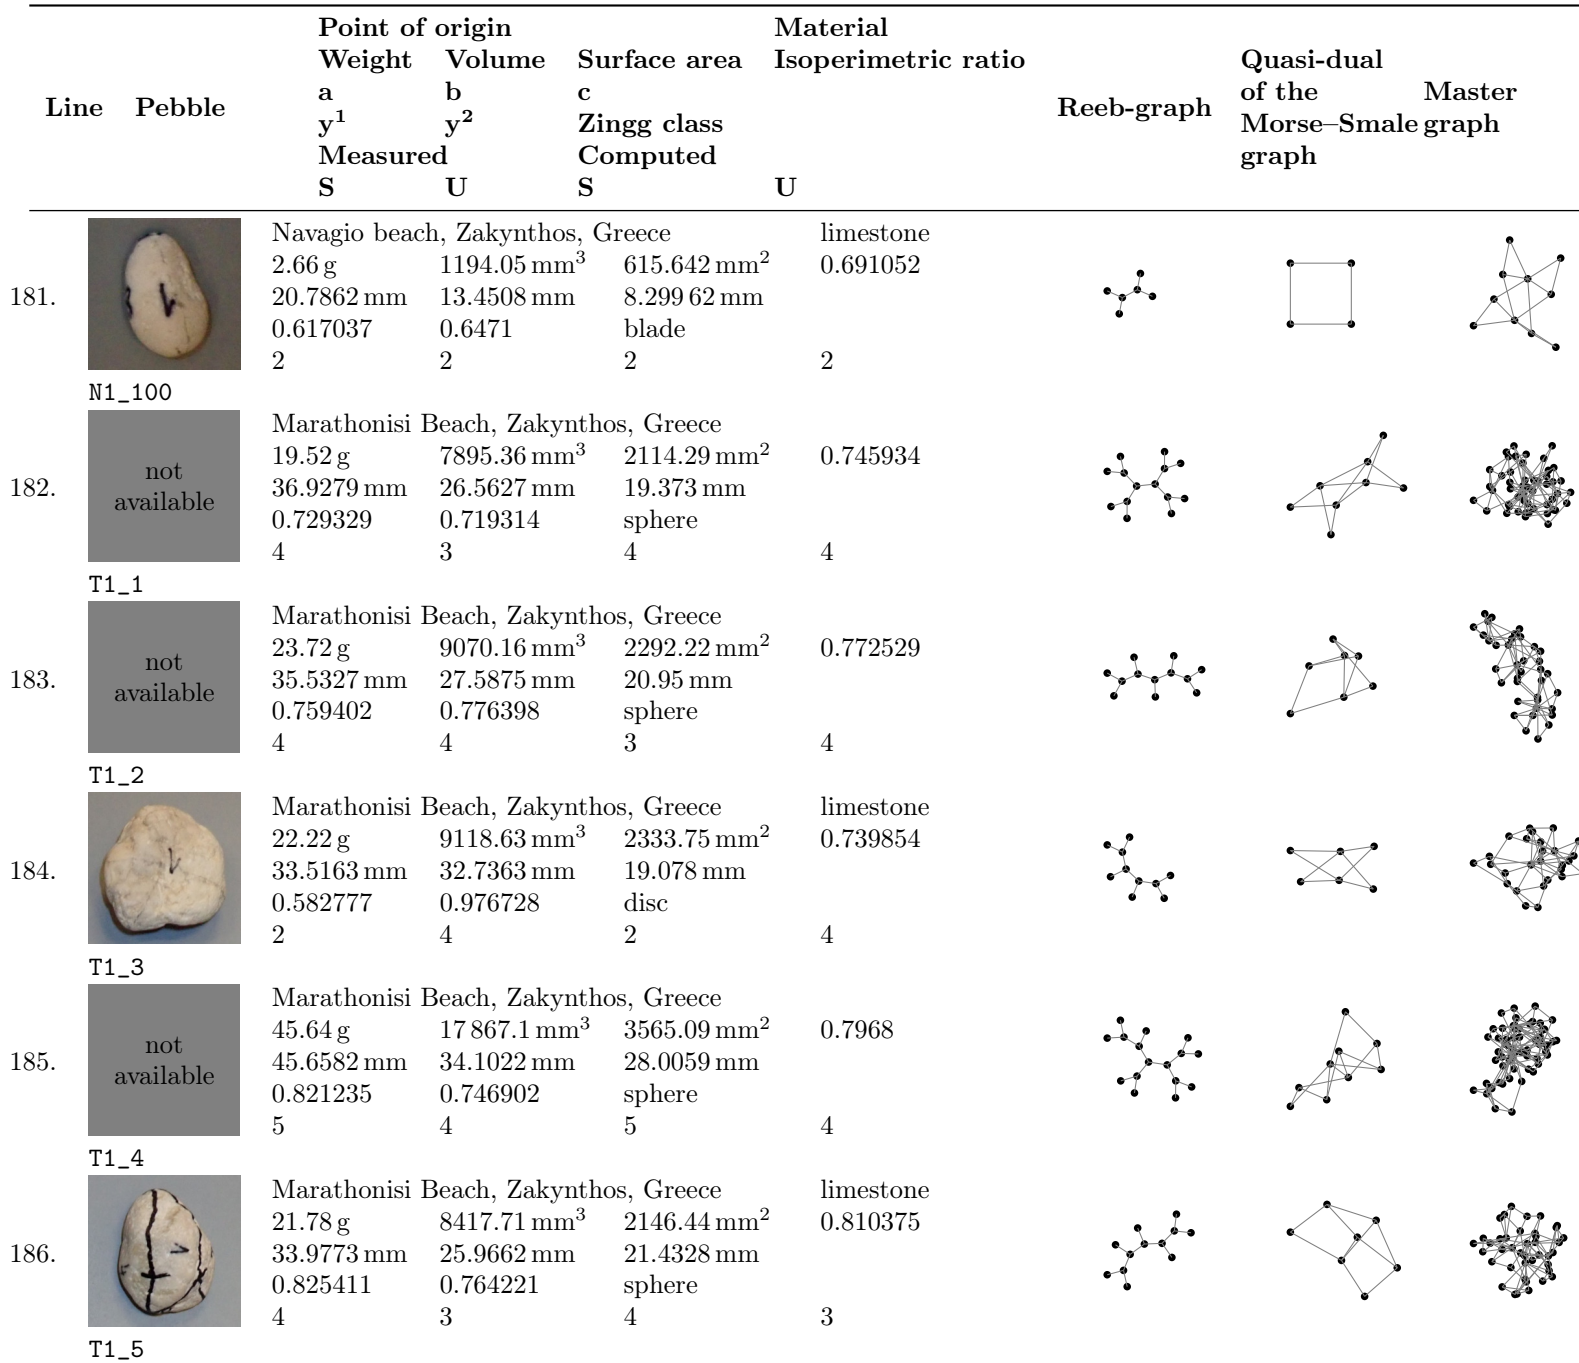  | 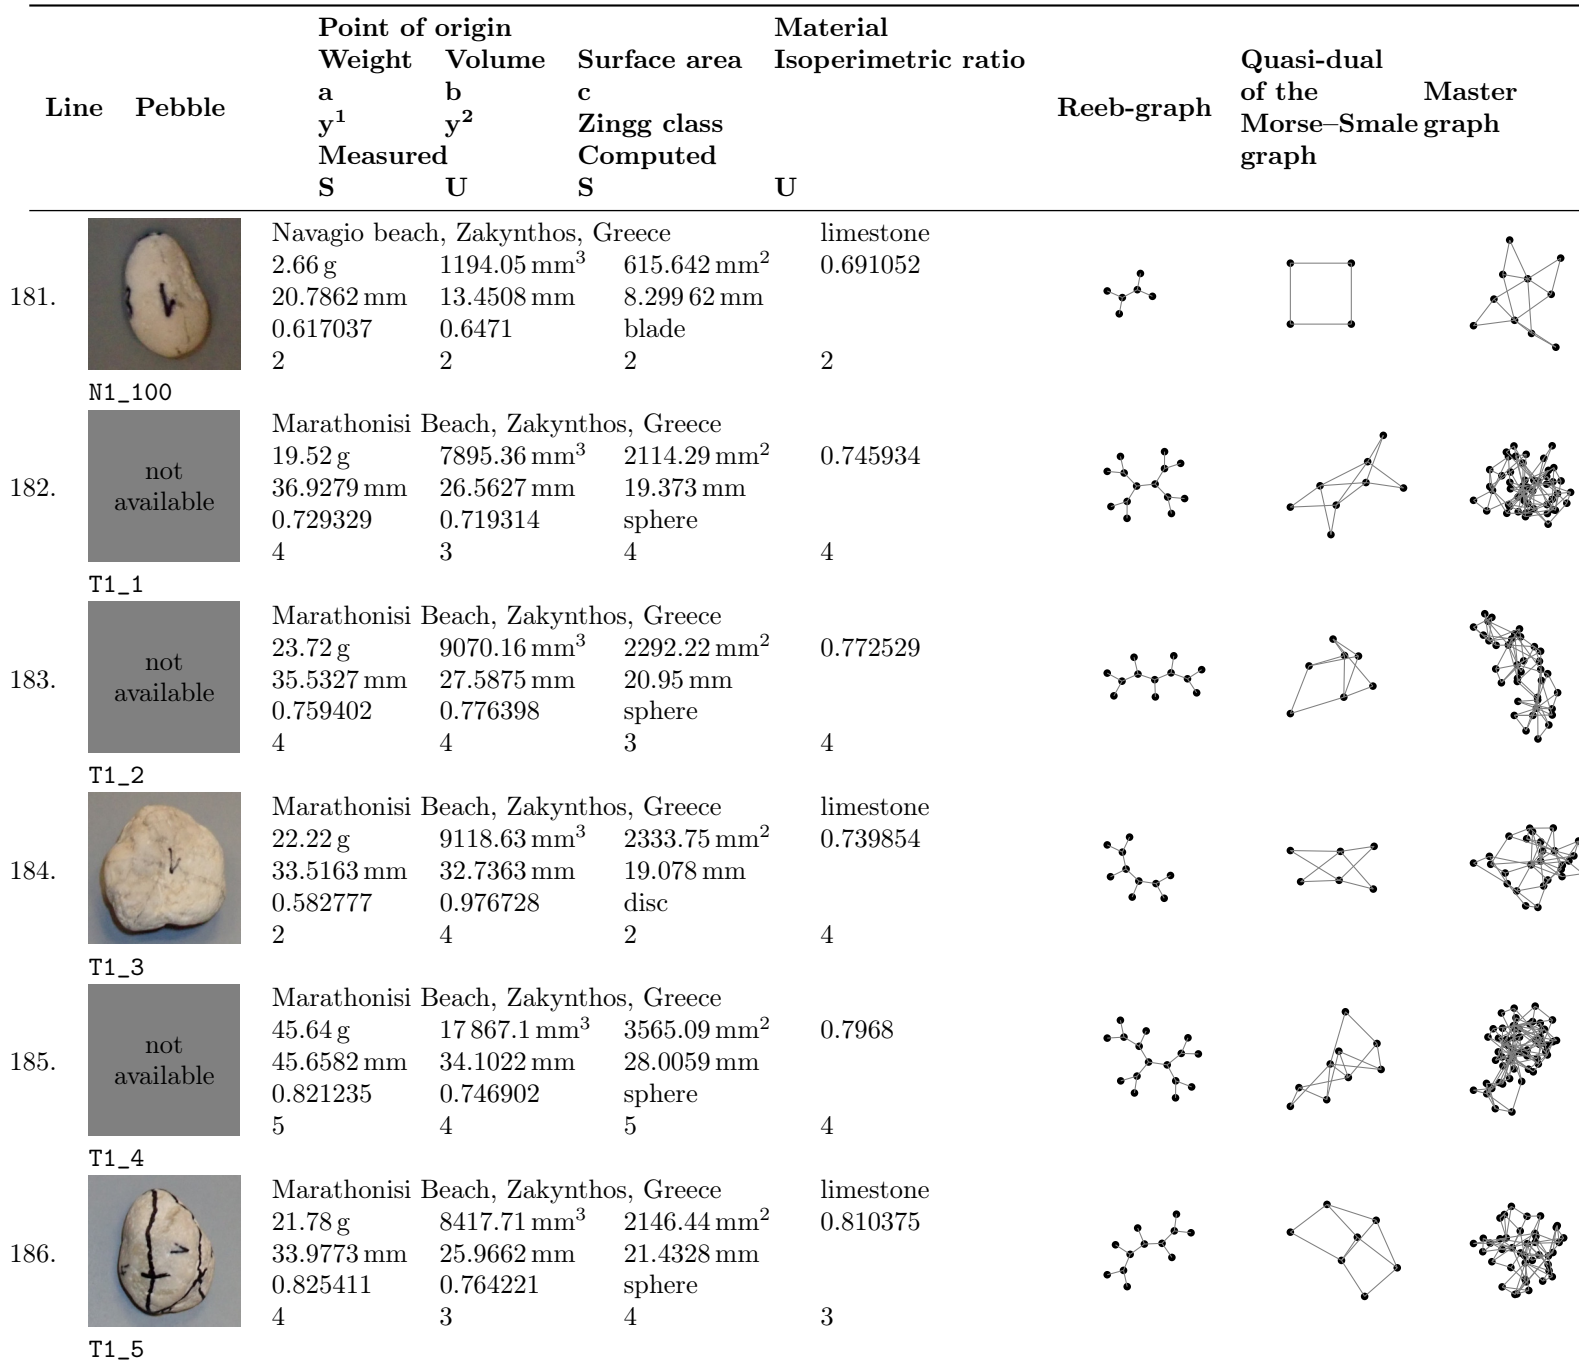  |
|      | T1_3                                                                                |                                                                                |                                                         |                                                      |                                |                                                                                       |                                                                                       |                                                                                       |
| 185. | 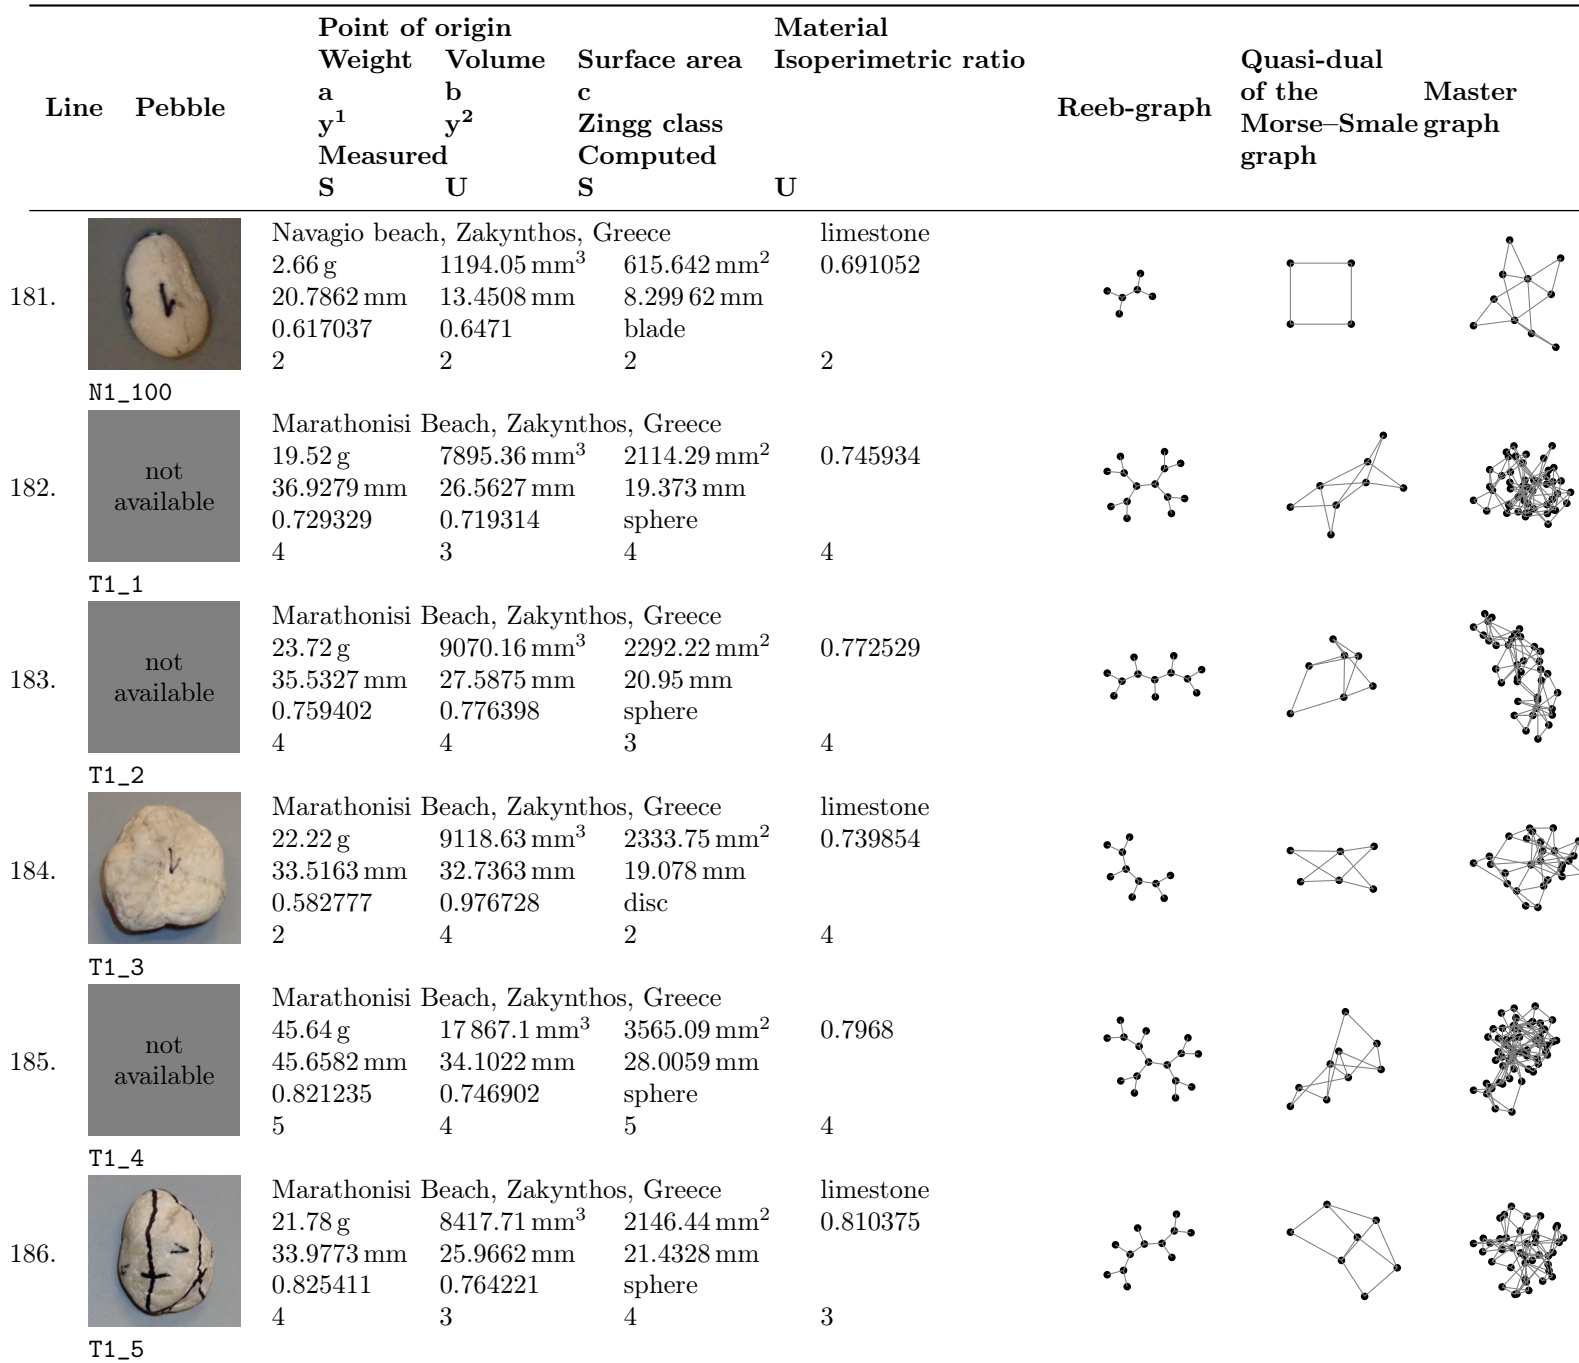 | Marathonisi Beach, Zakynthos, Greece<br>45.64 g<br>45.6582 mm<br>0.821235<br>5 | 17 867.1 mm <sup>3</sup><br>34.1022 mm<br>0.746902<br>4 | 3565.09 mm <sup>2</sup><br>28.0059 mm<br>sphere<br>5 | 0.7968<br><br>4                | 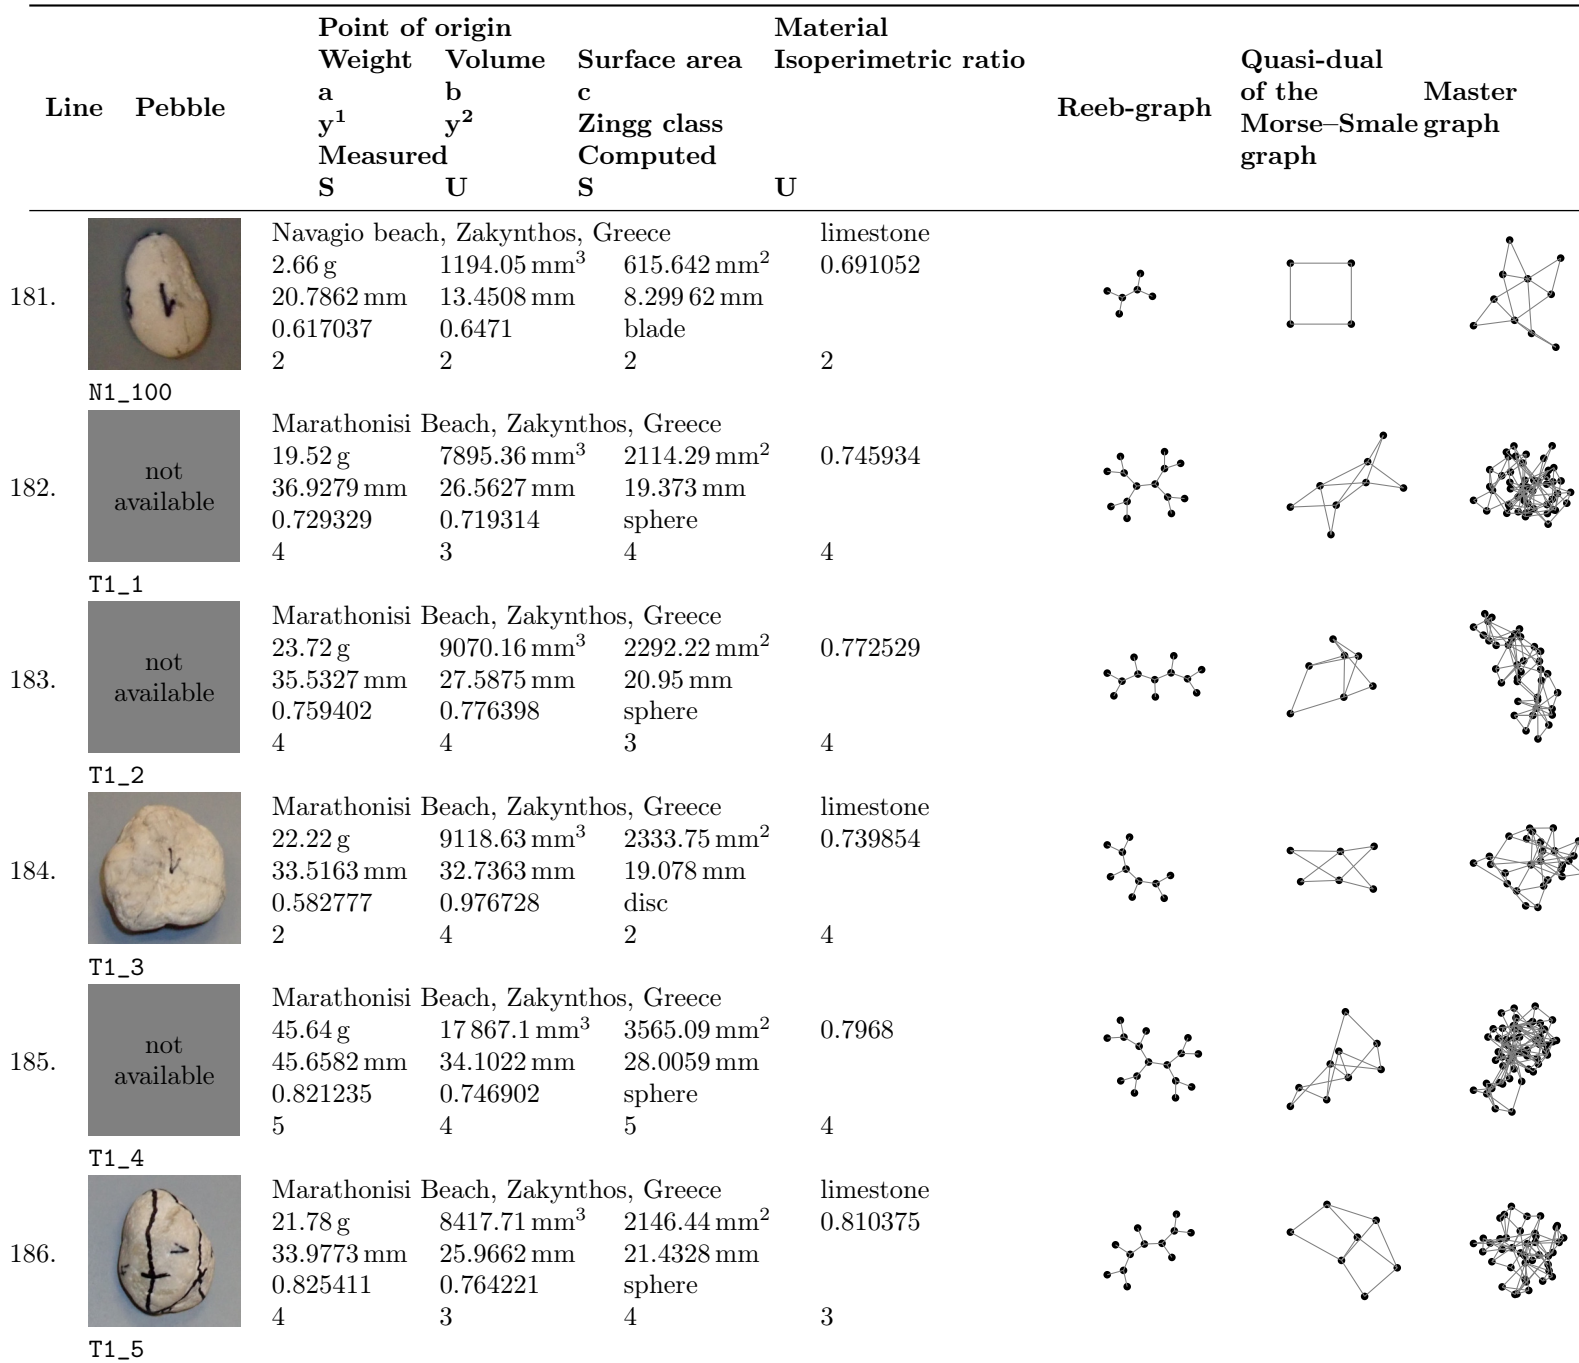 | 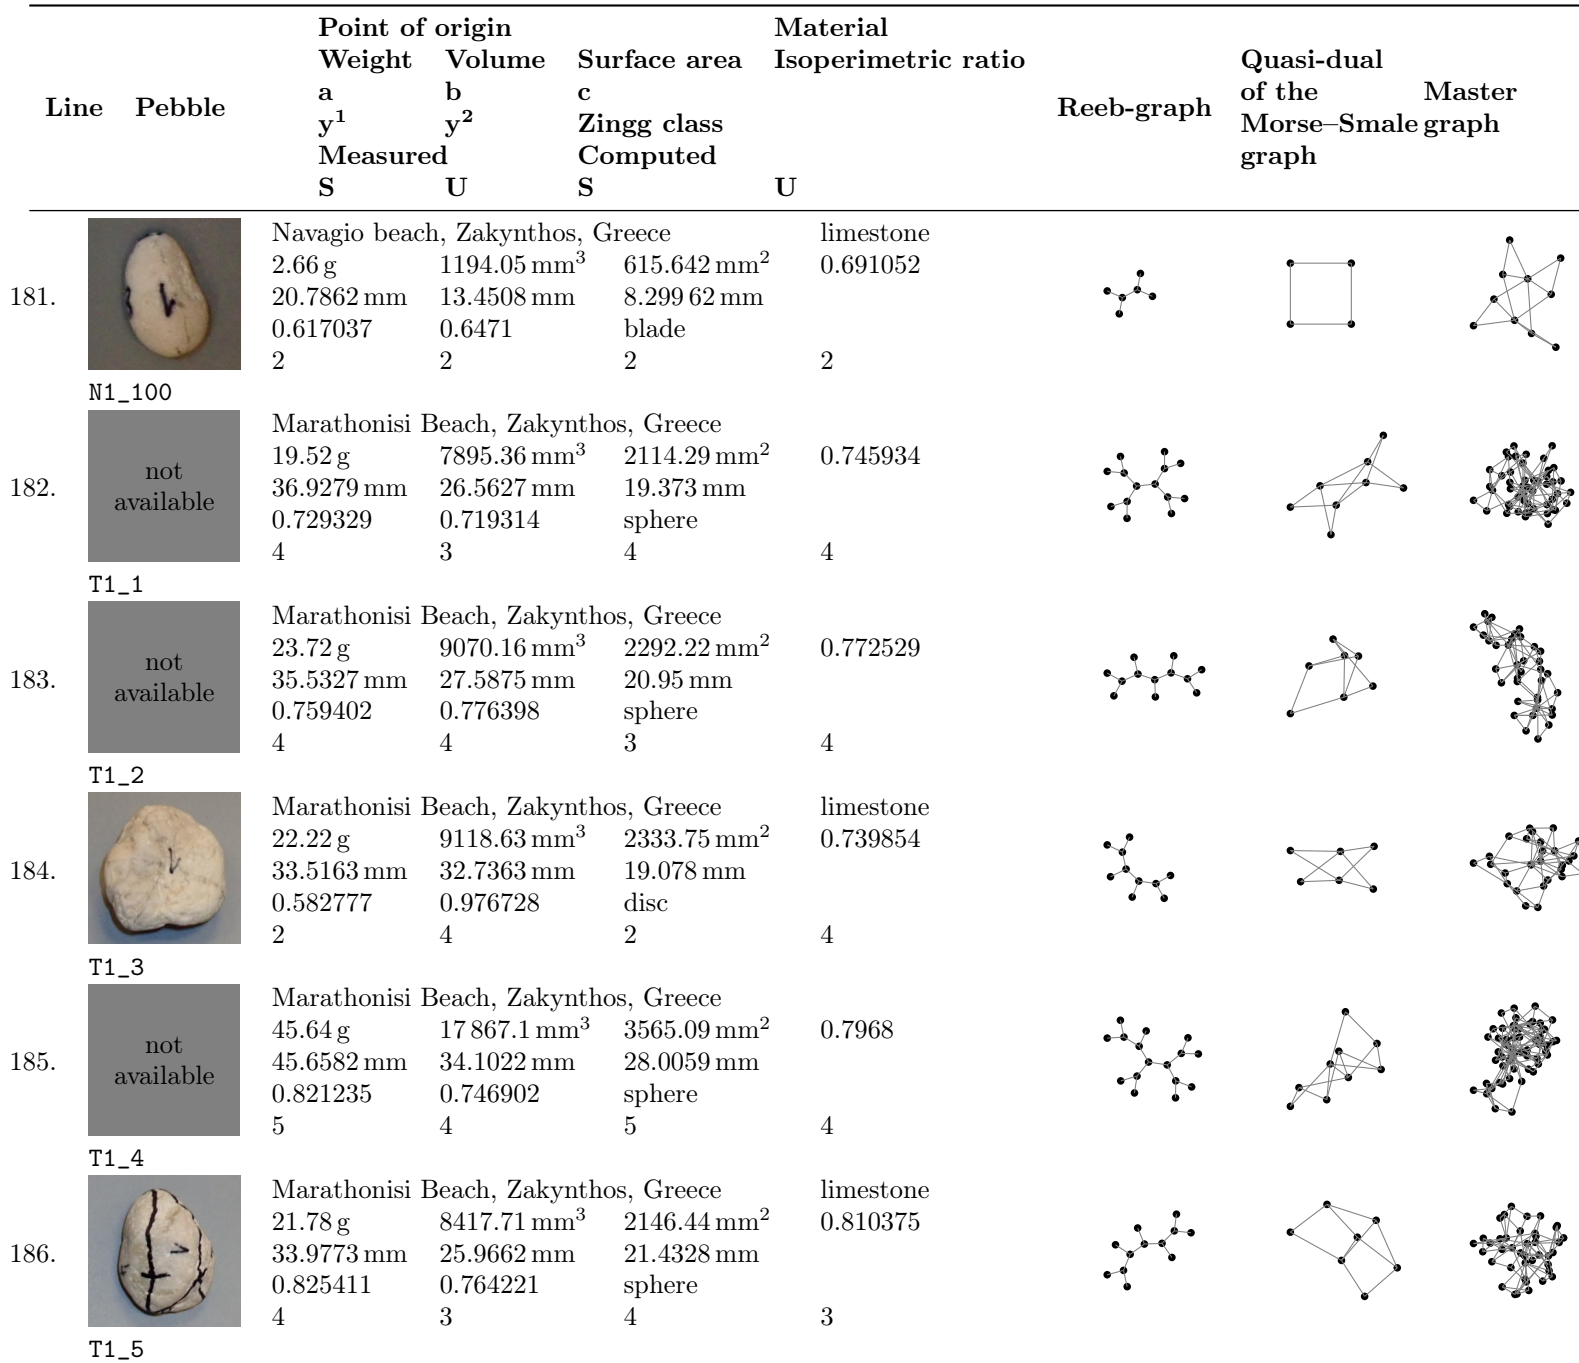 | 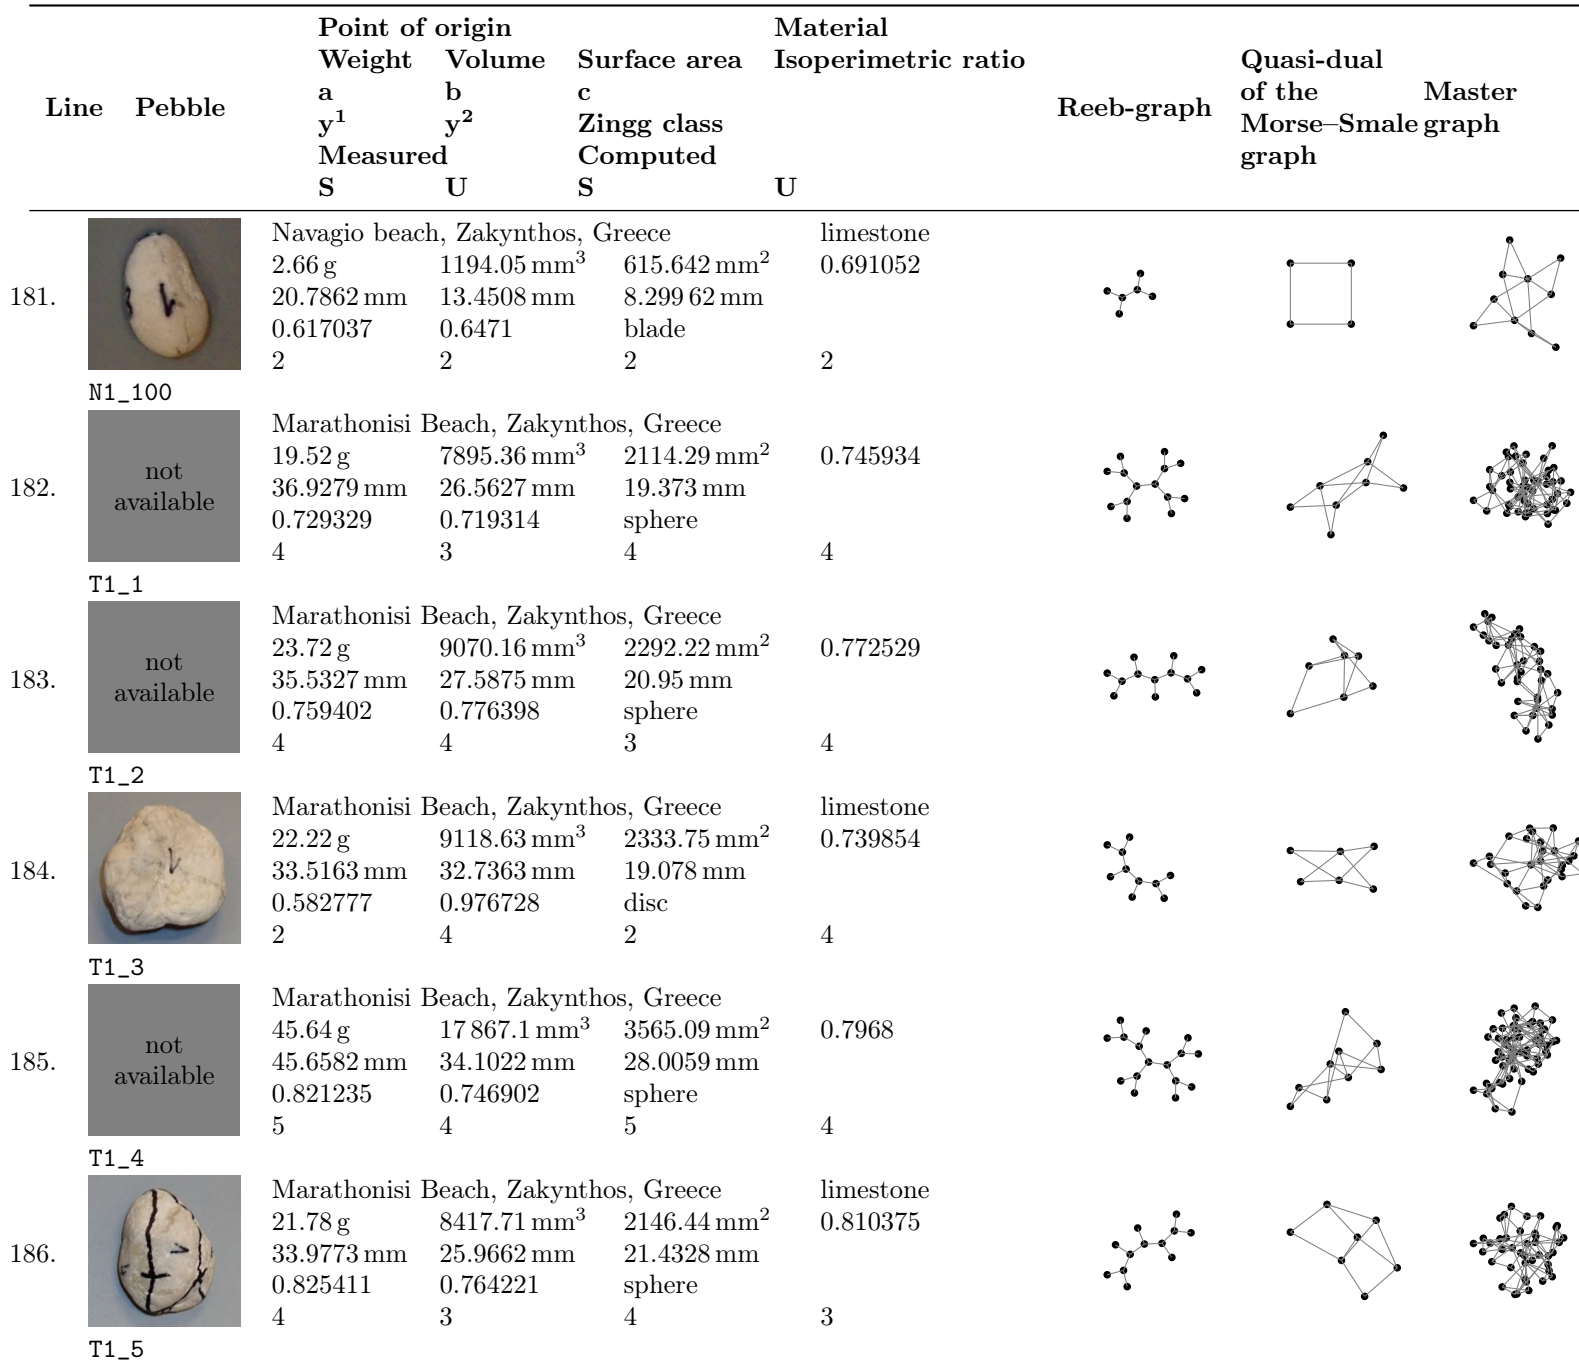 |
|      | T1_4                                                                                |                                                                                |                                                         |                                                      |                                |                                                                                       |                                                                                       |                                                                                       |
| 186. | 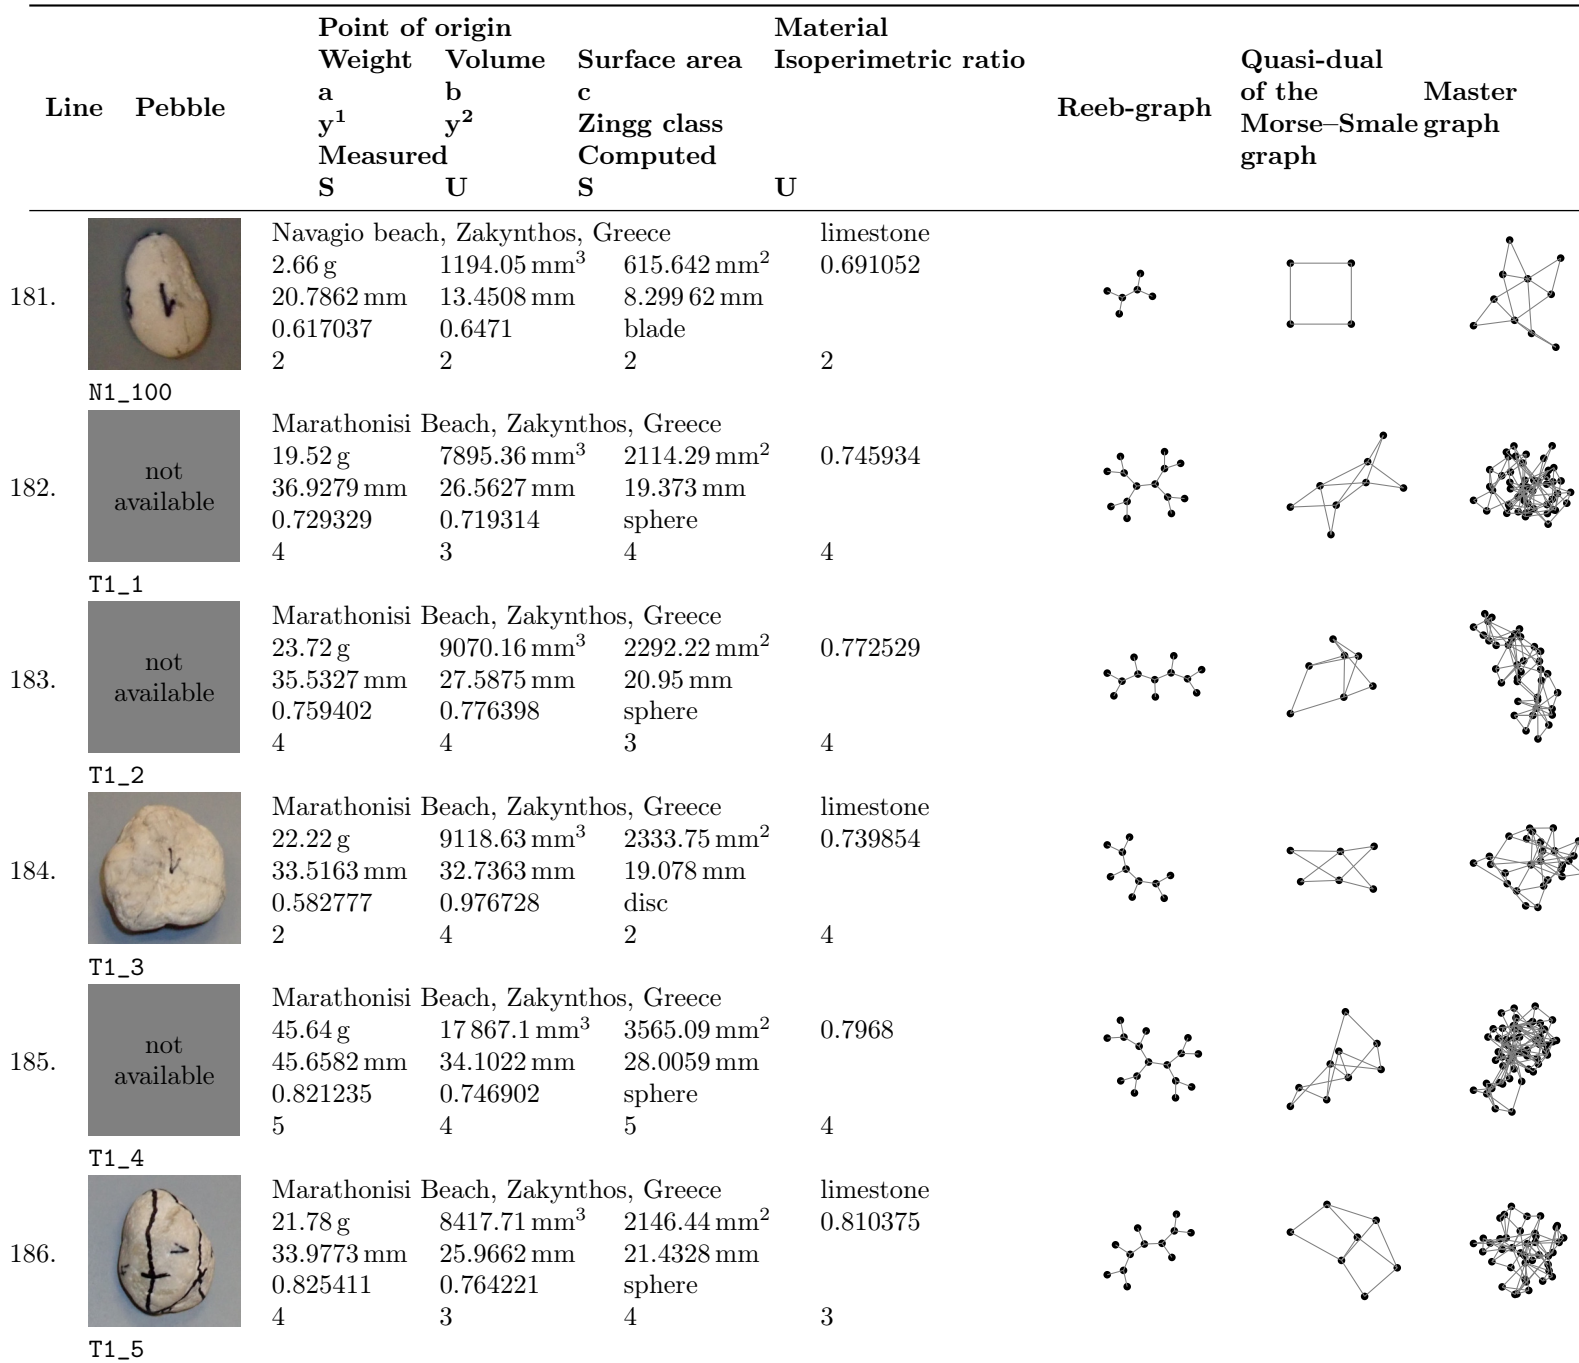 | Marathonisi Beach, Zakynthos, Greece<br>21.78 g<br>33.9773 mm<br>0.825411<br>4 | 8417.71 mm <sup>3</sup><br>25.9662 mm<br>0.764221<br>3  | 2146.44 mm <sup>2</sup><br>21.4328 mm<br>sphere<br>4 | limestone<br>0.810375<br><br>3 | 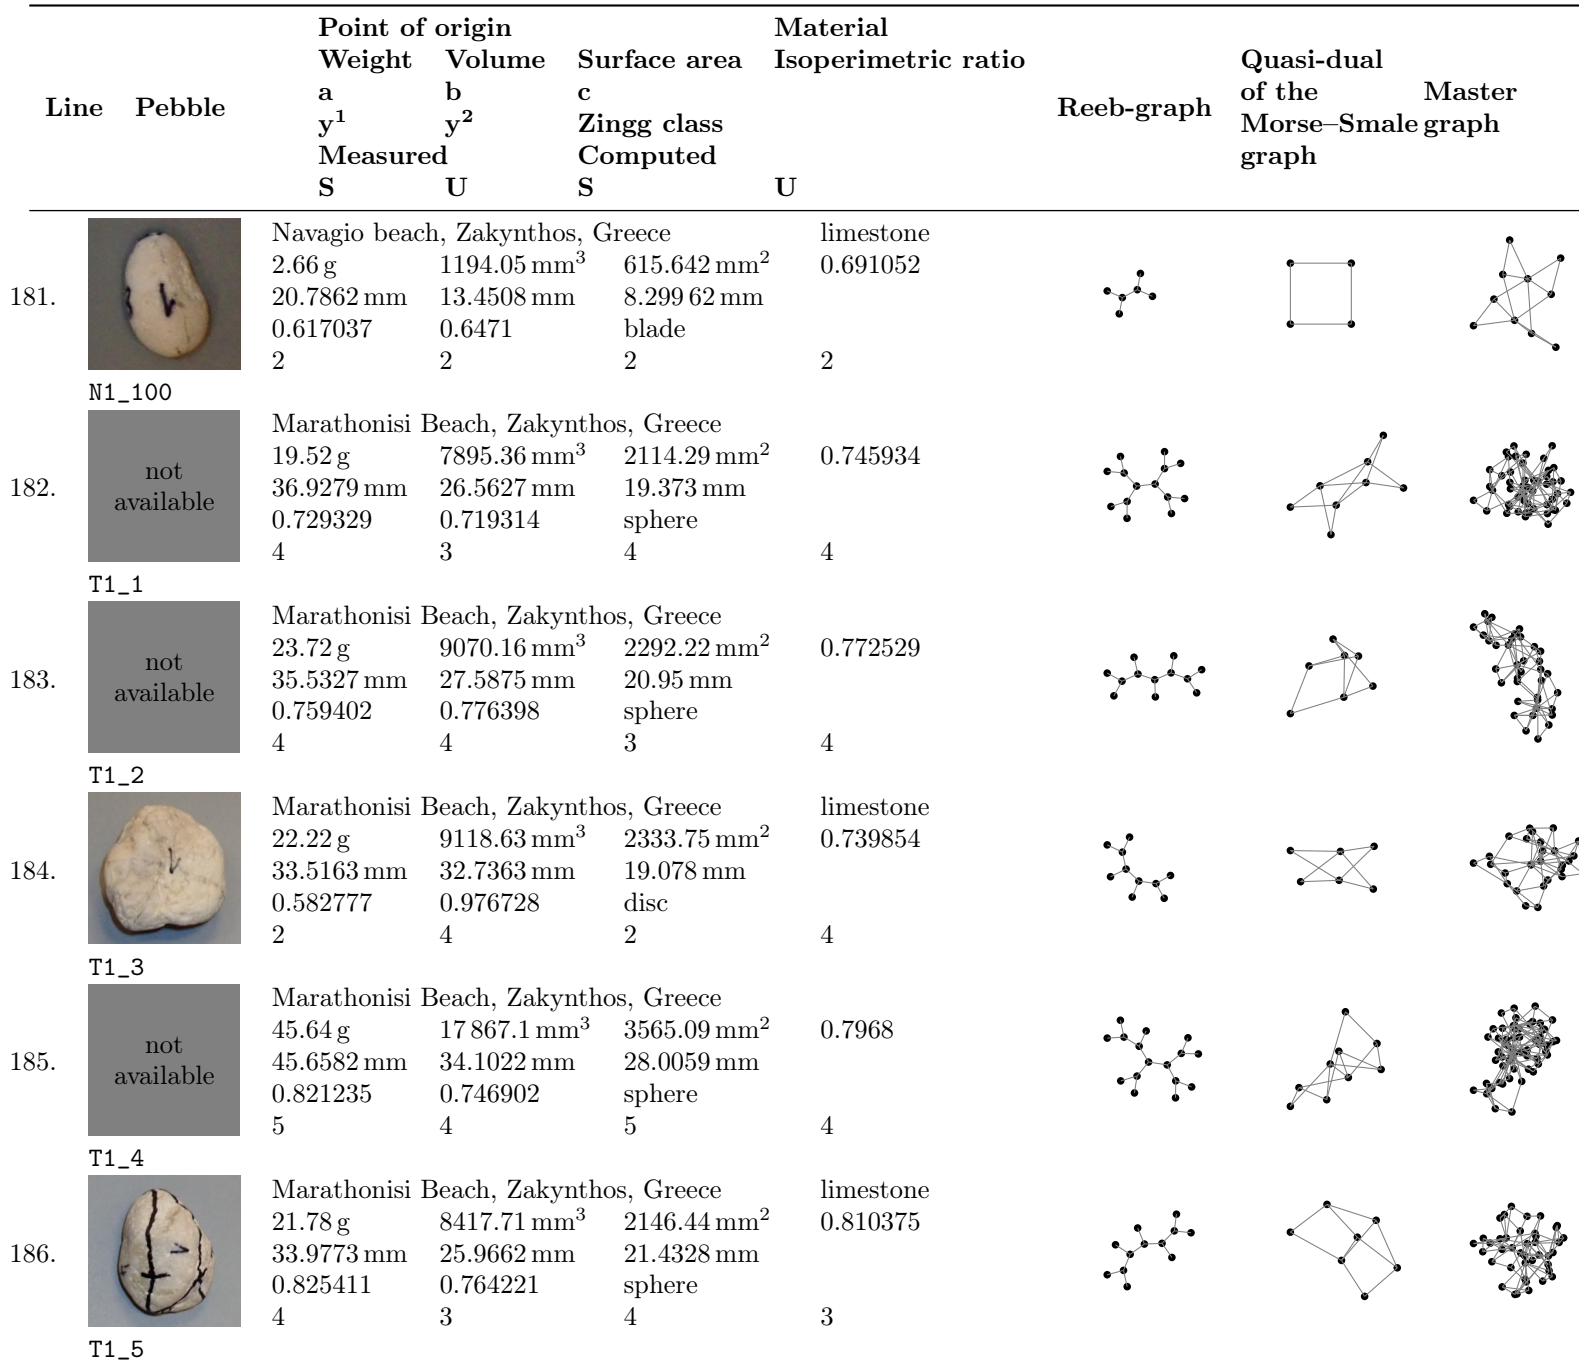 | 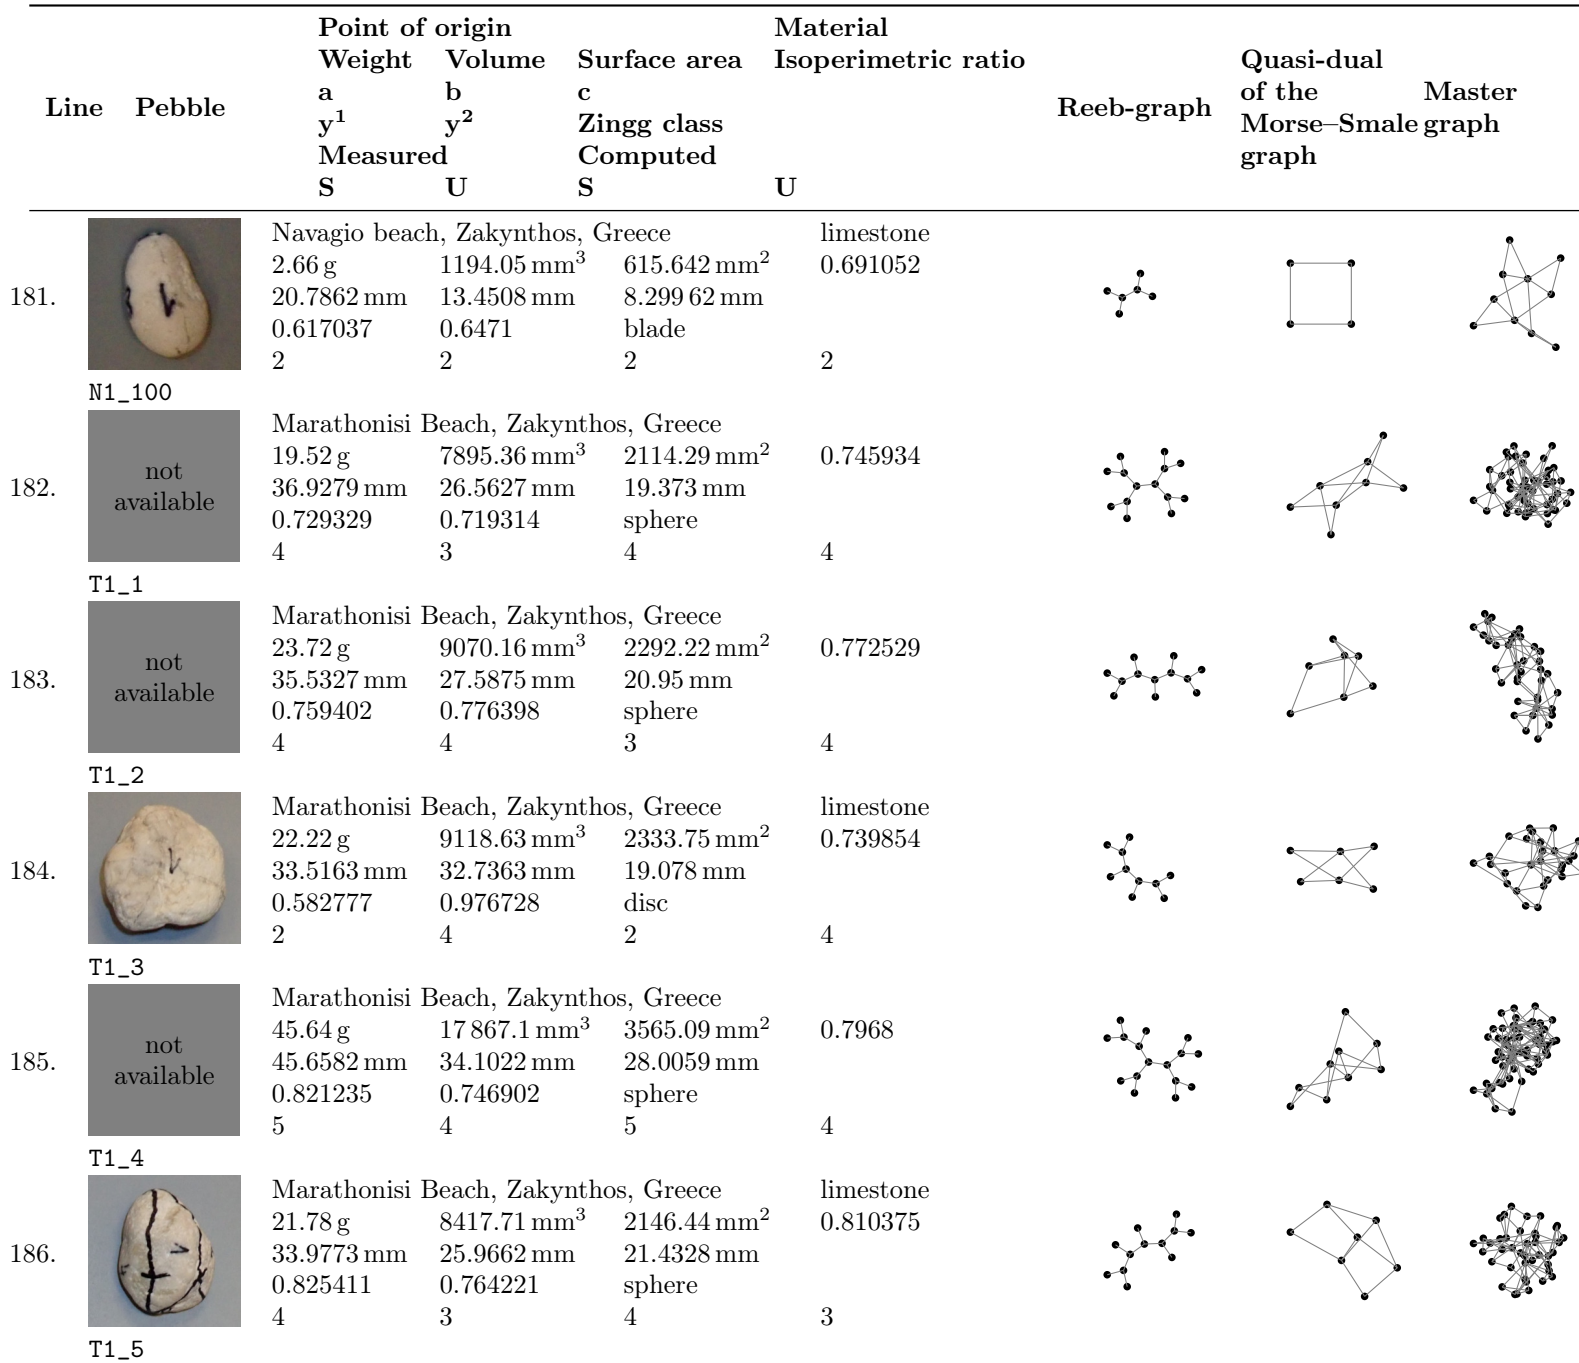 | 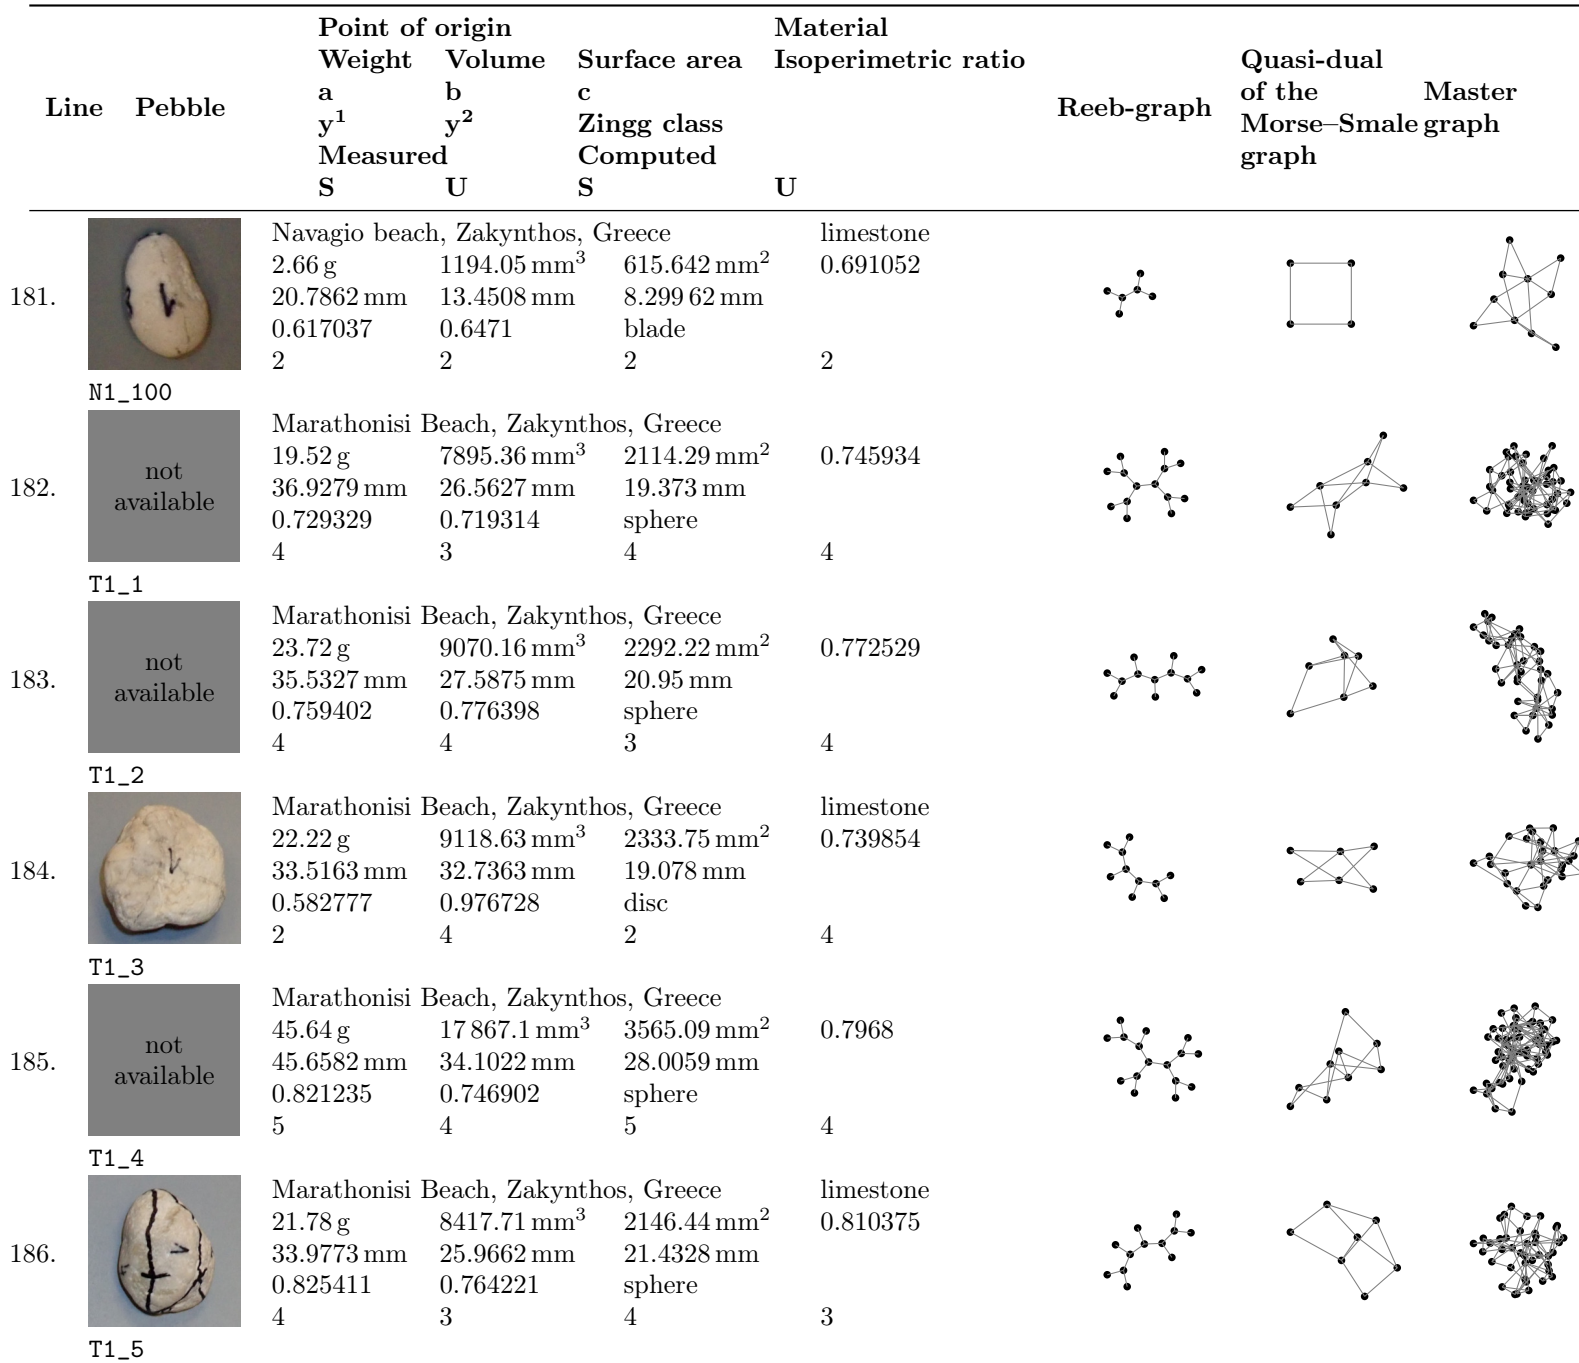 |
|      | T1_5                                                                                |                                                                                |                                                         |                                                      |                                |                                                                                       |                                                                                       |                                                                                       |

| Line  | Pebble                                                                              | Point of origin                                                                |                                                         | Surface area<br>c<br>Zingg class<br>Computed<br>S    | Material<br>Isoperimetric ratio<br>U | Reeb-graph                                                                            | Quasi-dual<br>of the<br>Morse–Smale<br>graph                                          | Master<br>graph                                                                       |
|-------|-------------------------------------------------------------------------------------|--------------------------------------------------------------------------------|---------------------------------------------------------|------------------------------------------------------|--------------------------------------|---------------------------------------------------------------------------------------|---------------------------------------------------------------------------------------|---------------------------------------------------------------------------------------|
|       |                                                                                     | Weight                                                                         | Volume                                                  |                                                      |                                      |                                                                                       |                                                                                       |                                                                                       |
|       |                                                                                     | a<br>y <sup>1</sup><br>Measured<br>S                                           | b<br>y <sup>2</sup><br>U                                |                                                      |                                      |                                                                                       |                                                                                       |                                                                                       |
|       |                                                                                     |                                                                                |                                                         |                                                      |                                      |                                                                                       |                                                                                       |                                                                                       |
| 187.  | 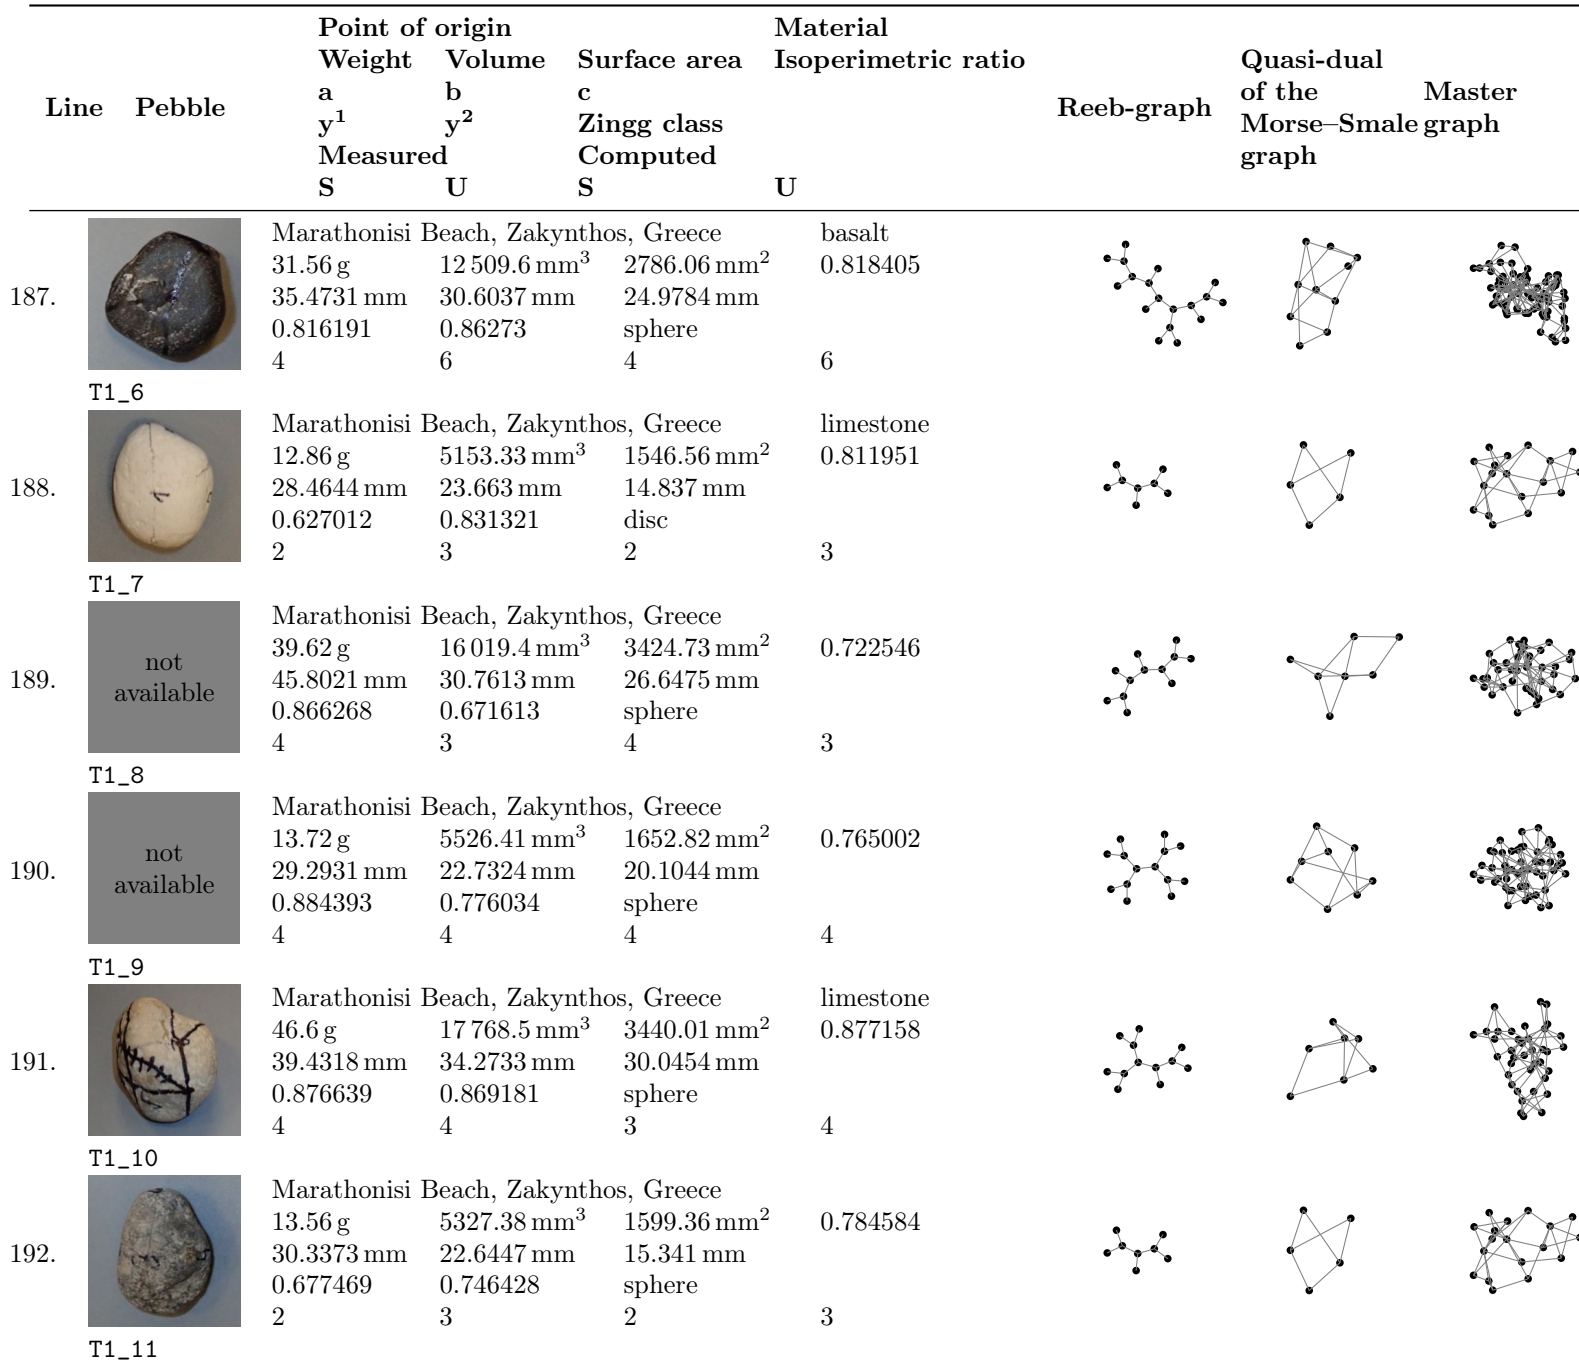   | Marathonisi Beach, Zakynthos, Greece<br>31.56 g<br>35.4731 mm<br>0.816191<br>4 | 3278.6 mm <sup>3</sup><br>30.6037 mm<br>0.86273<br>6    | 2786.06 mm <sup>2</sup><br>24.9784 mm<br>sphere<br>4 | basalt<br>0.818405<br><br>6          | 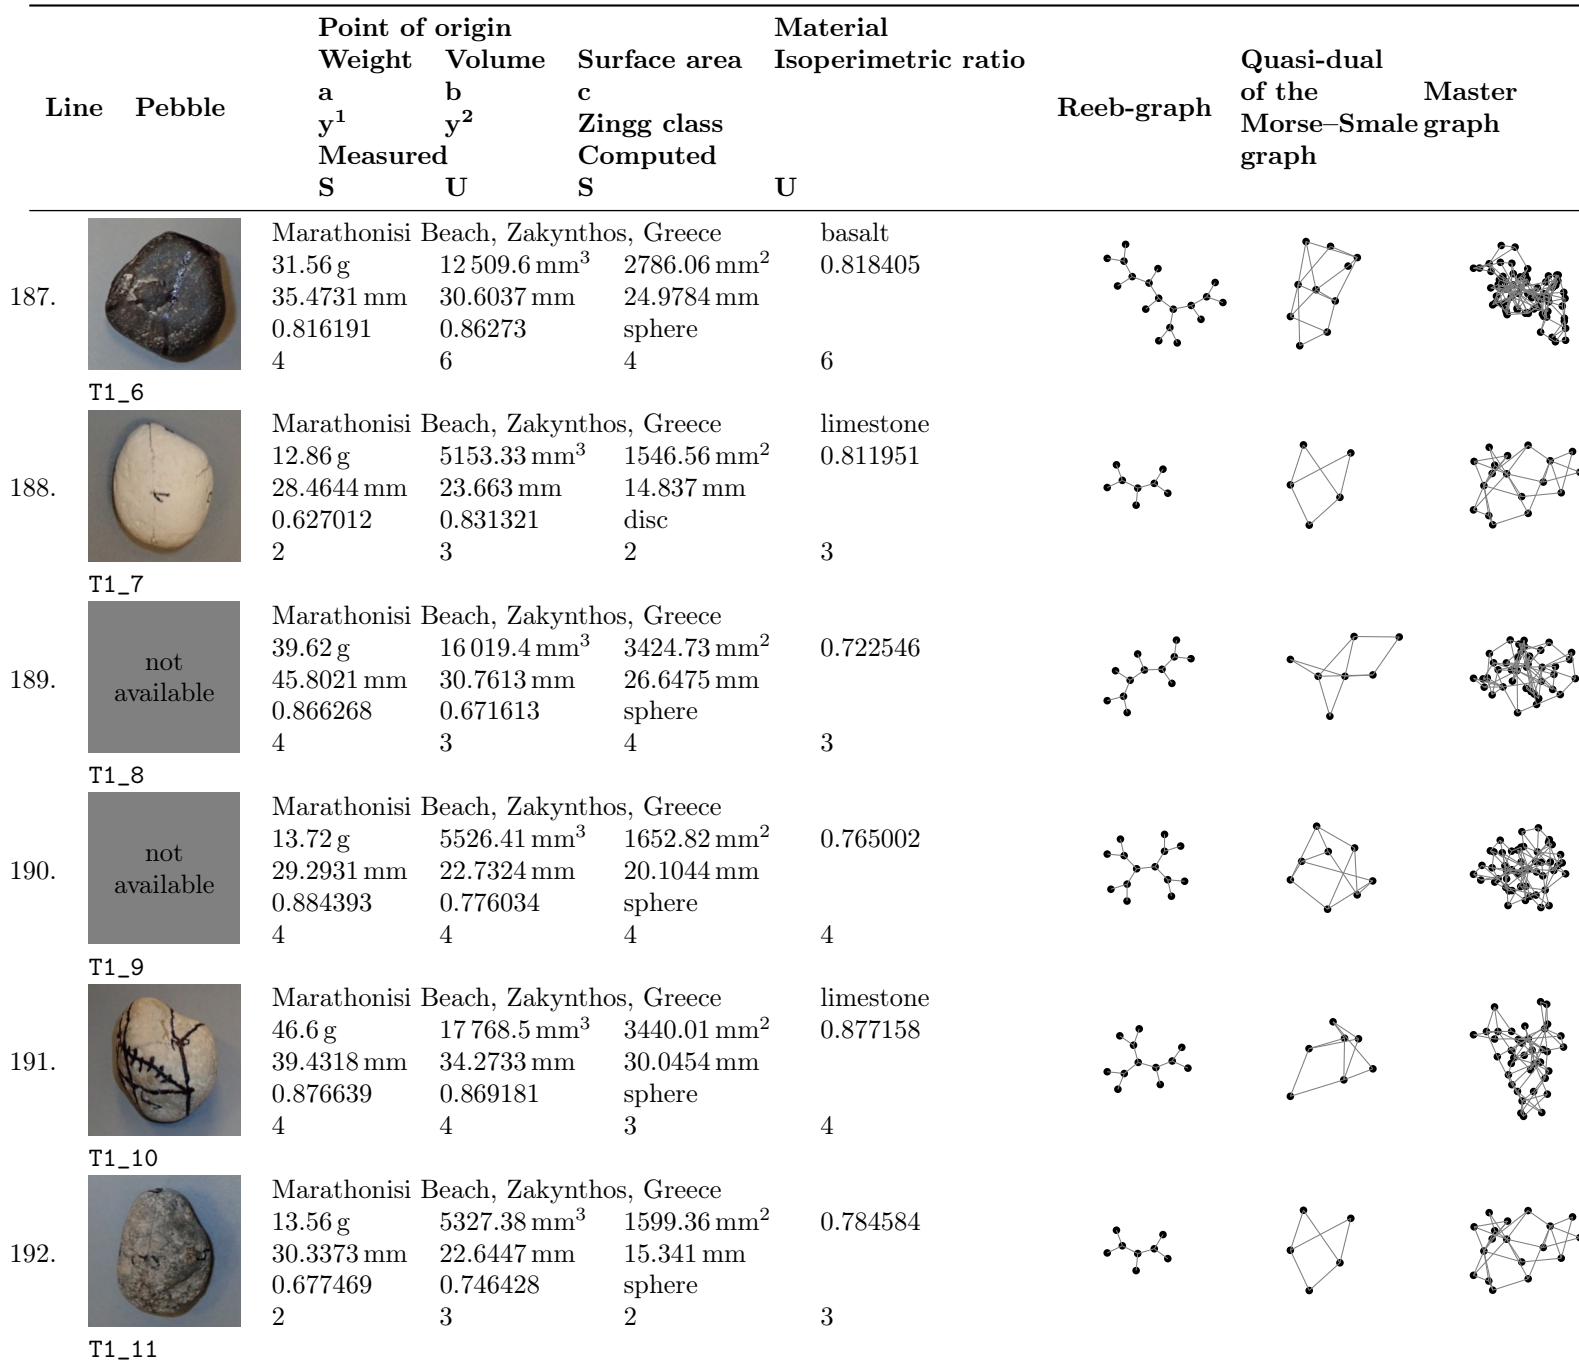   | 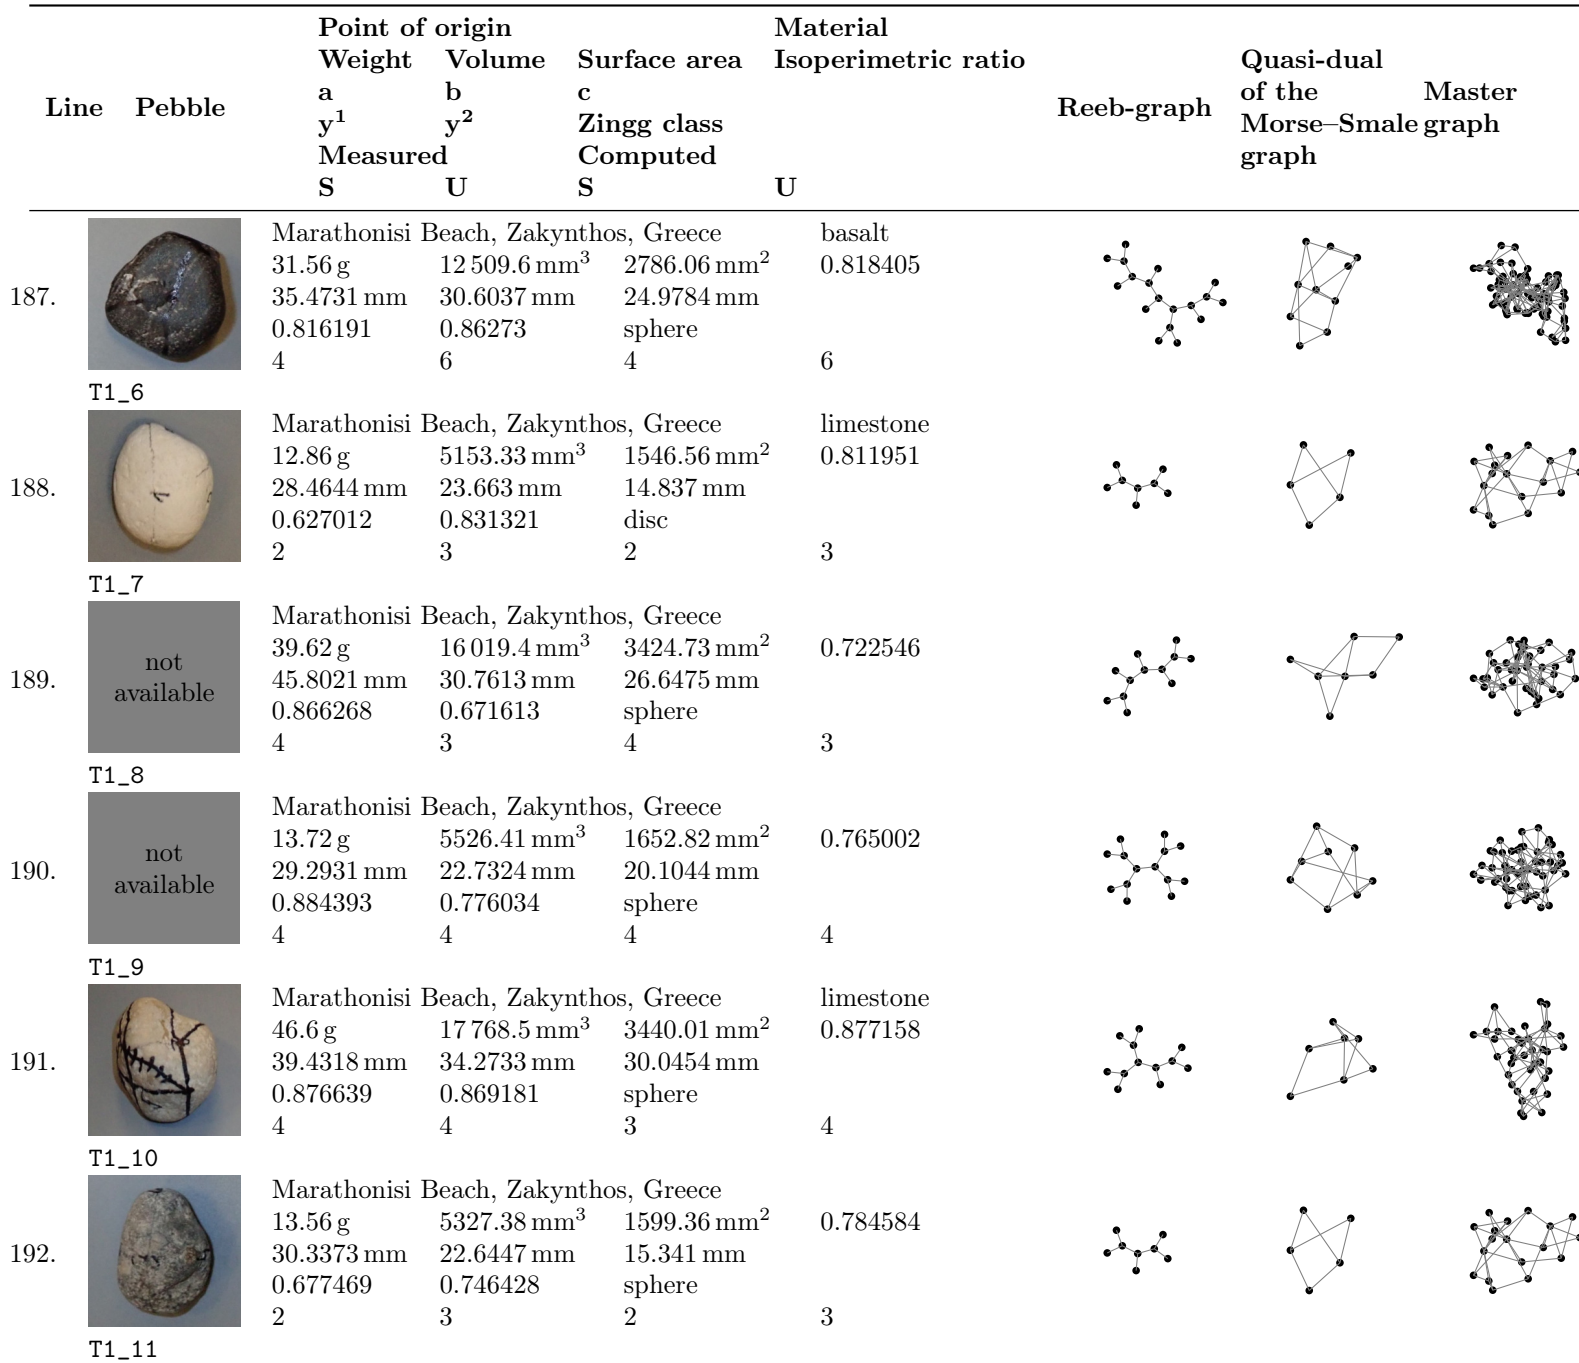   | 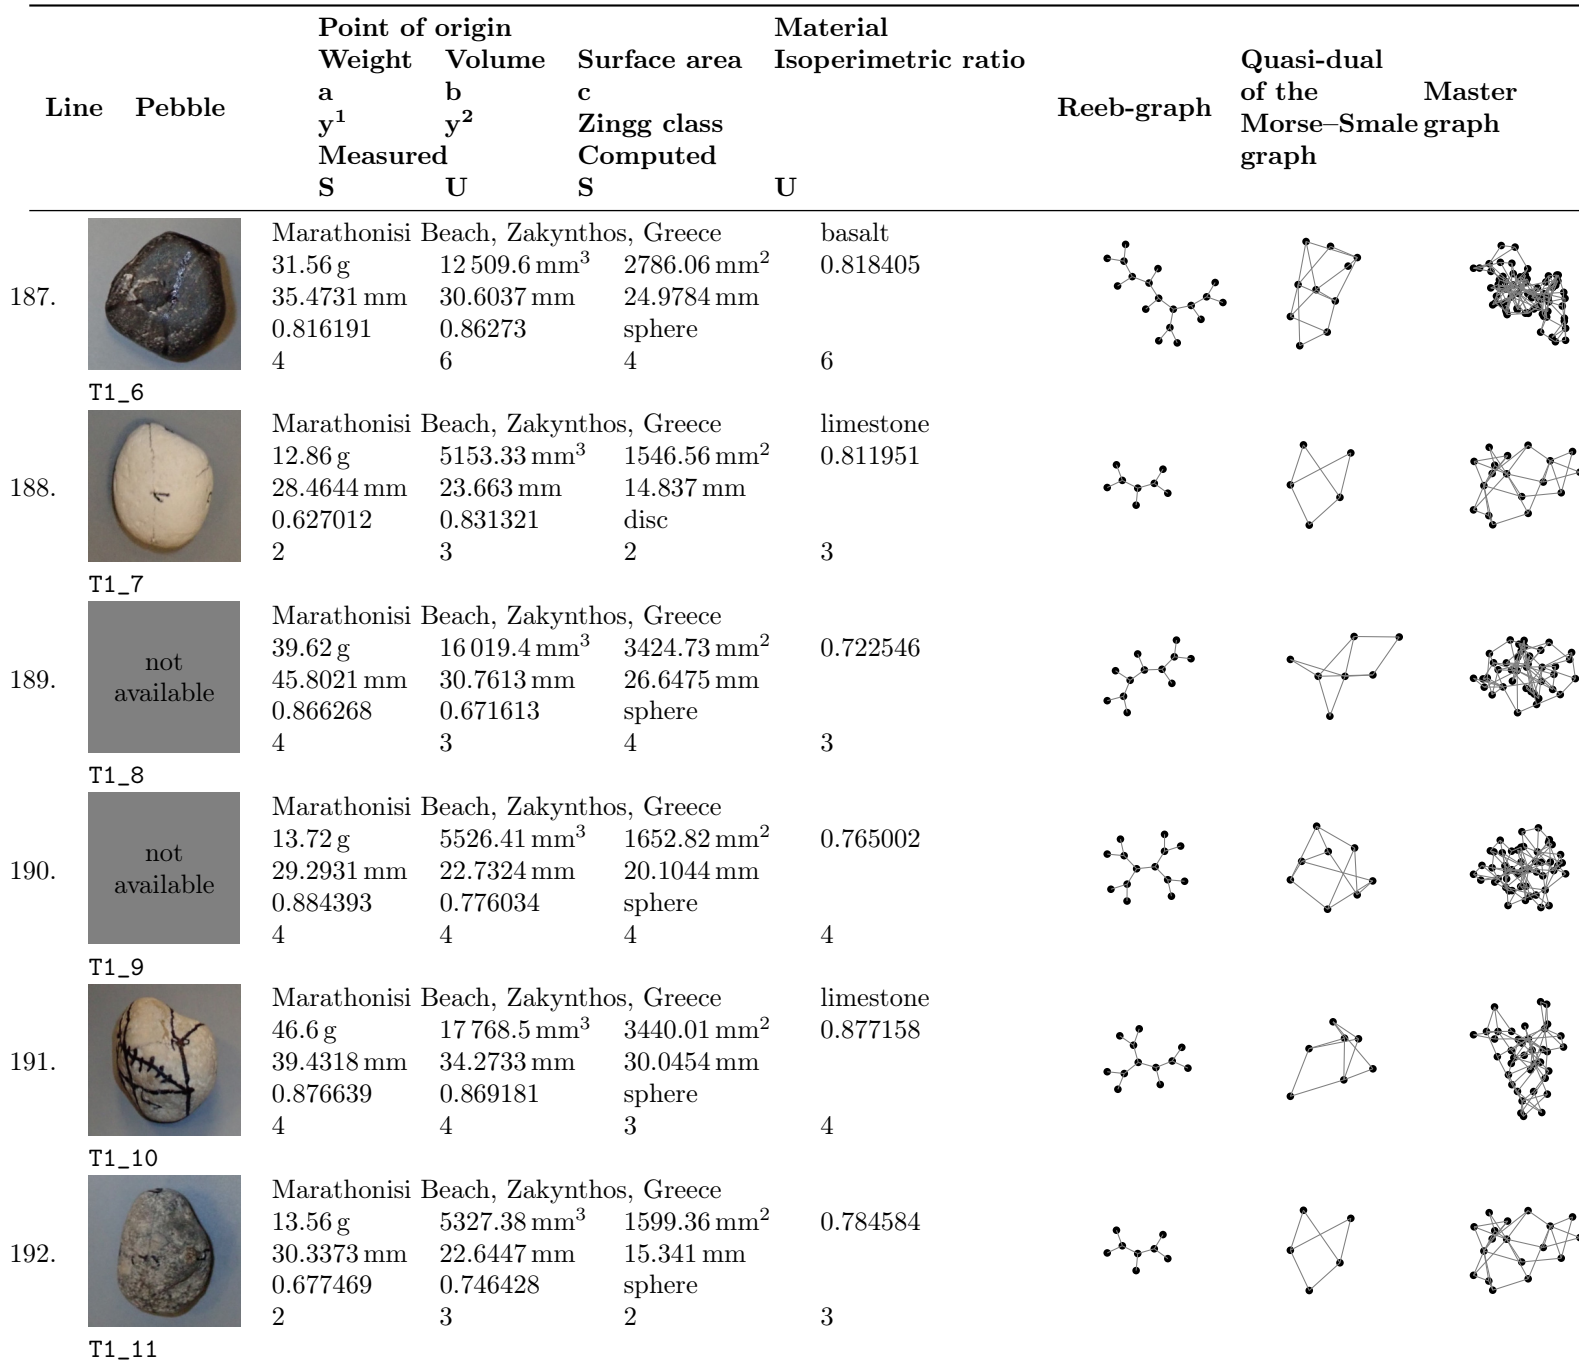   |
| T1_6  |                                                                                     |                                                                                |                                                         |                                                      |                                      |                                                                                       |                                                                                       |                                                                                       |
| 188.  | 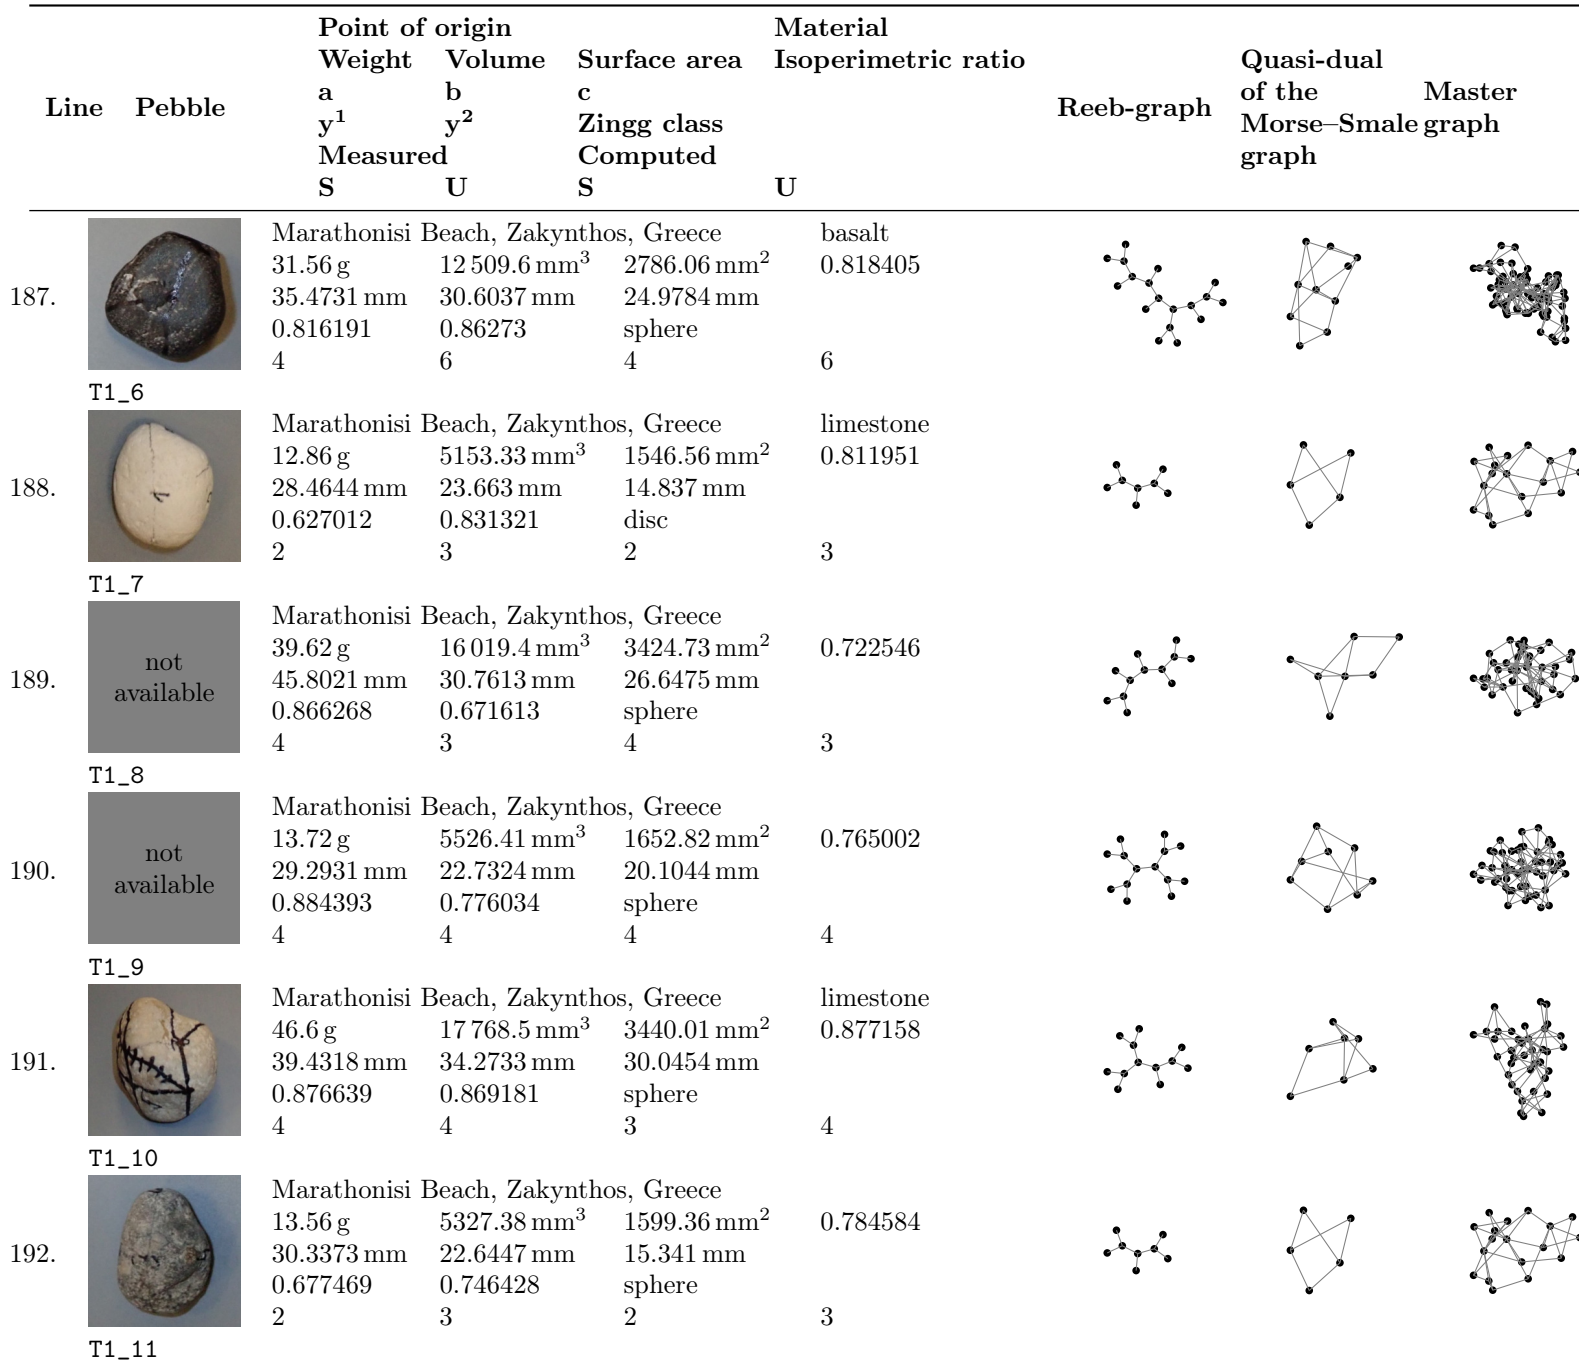   | Marathonisi Beach, Zakynthos, Greece<br>12.86 g<br>28.4644 mm<br>0.627012<br>2 | 5153.33 mm <sup>3</sup><br>23.663 mm<br>0.831321<br>3   | 1546.56 mm <sup>2</sup><br>14.837 mm<br>disc<br>2    | limestone<br>0.811951<br><br>3       | 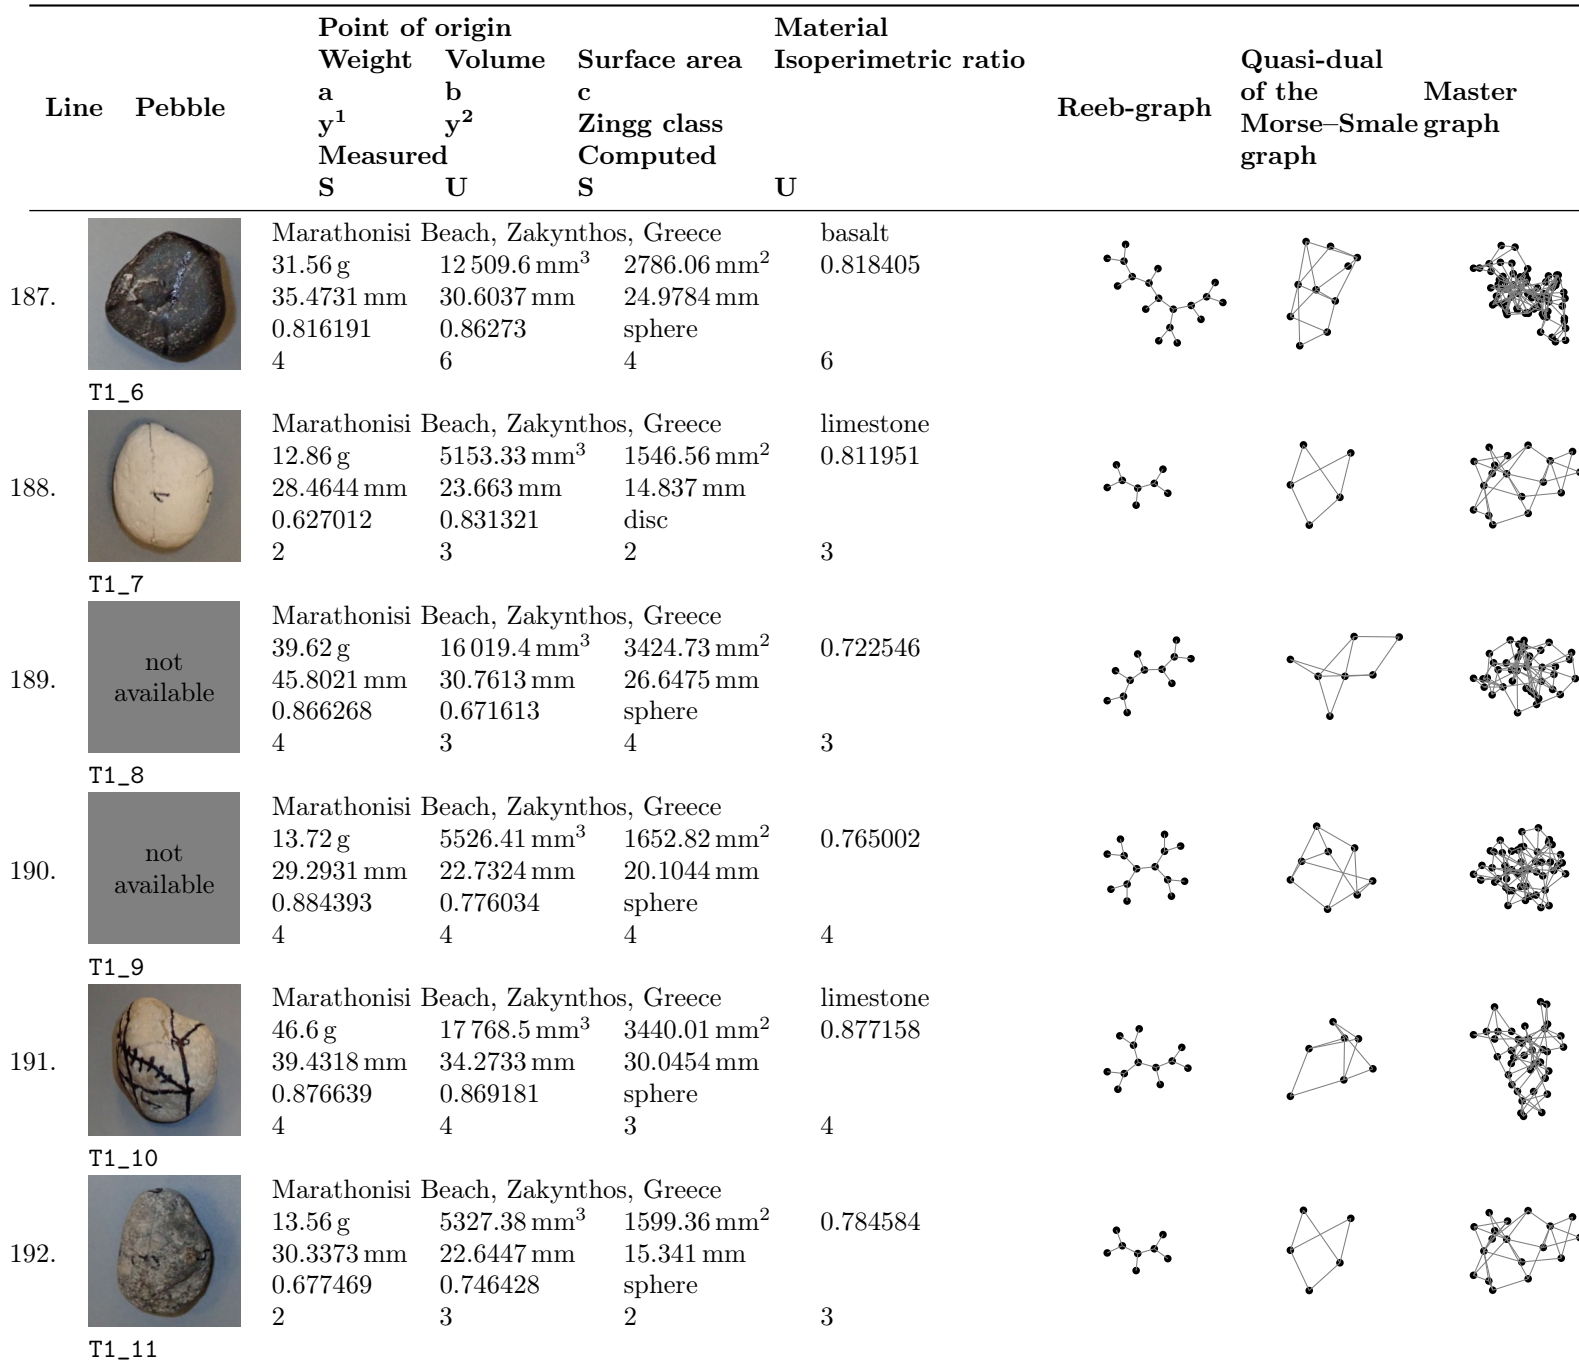   | 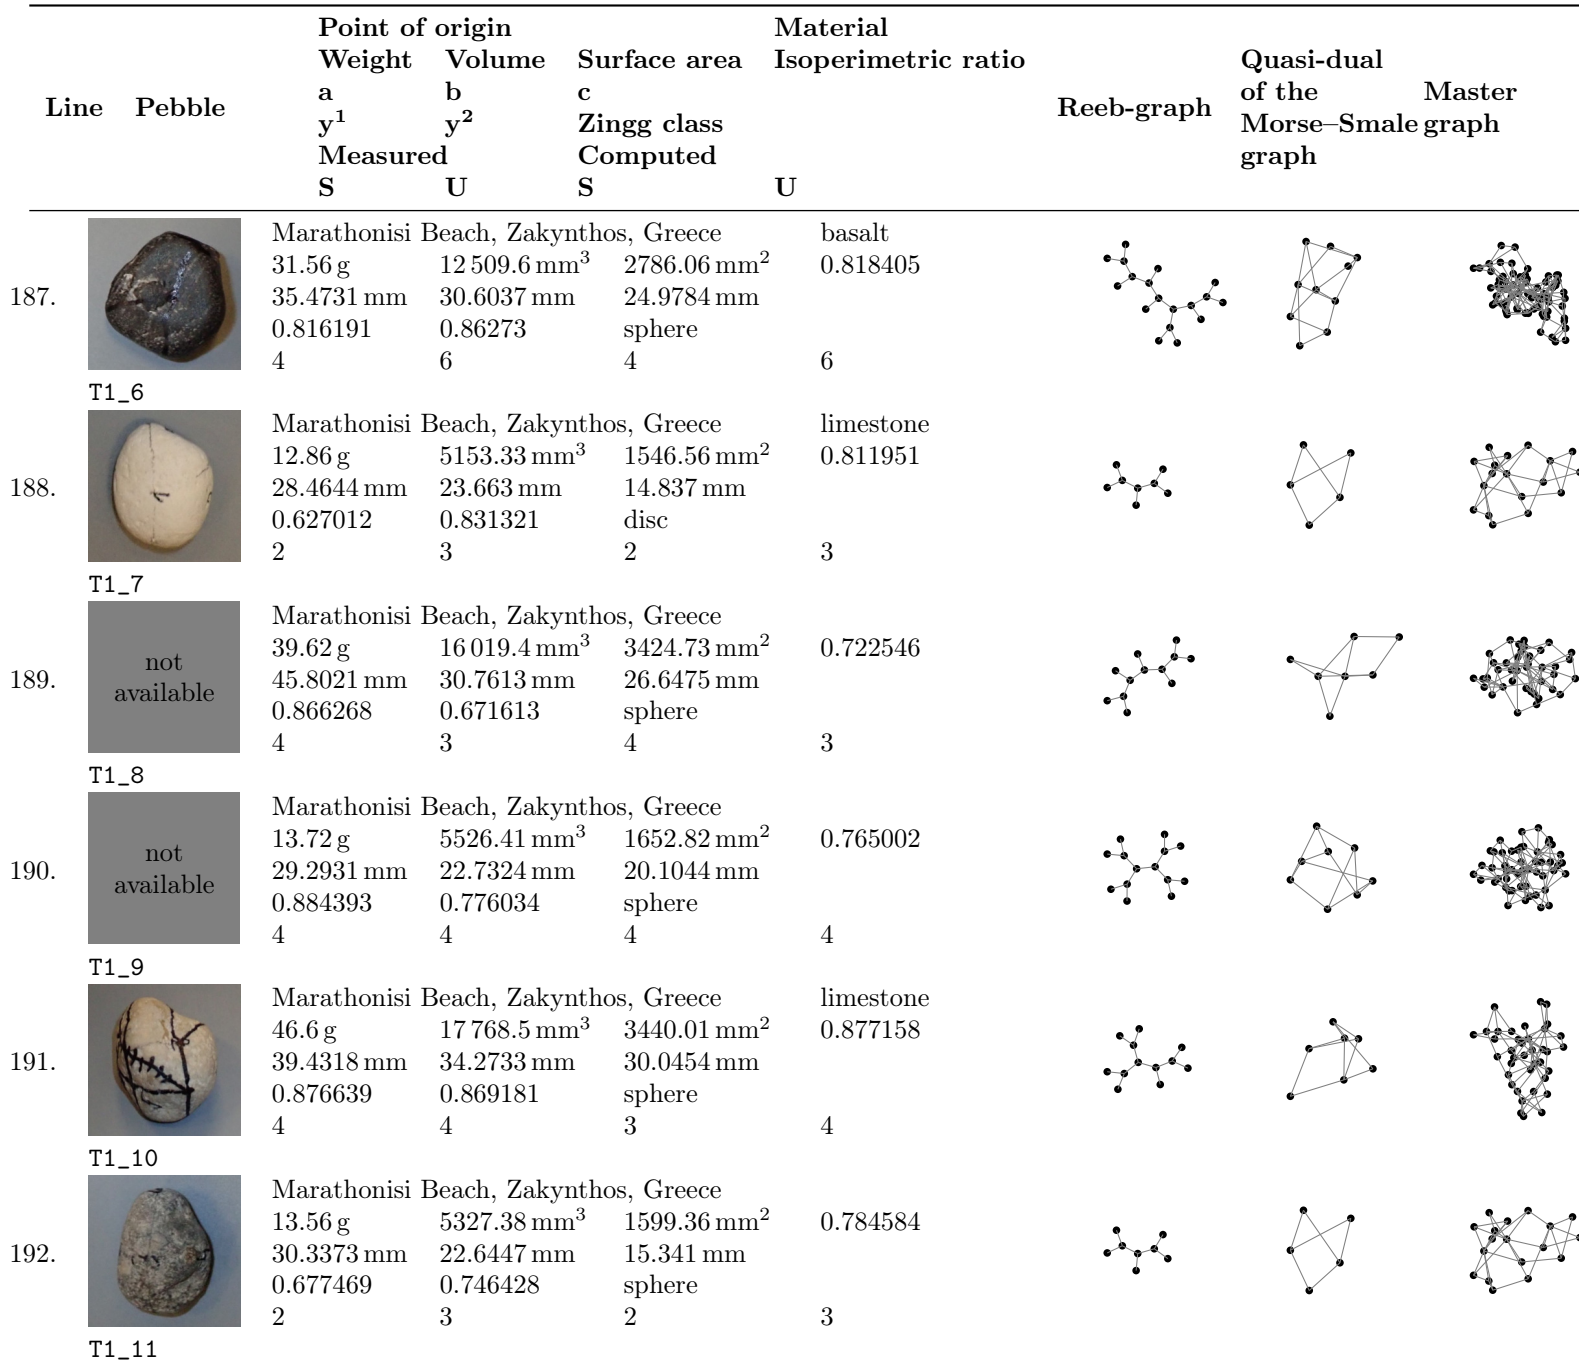   | 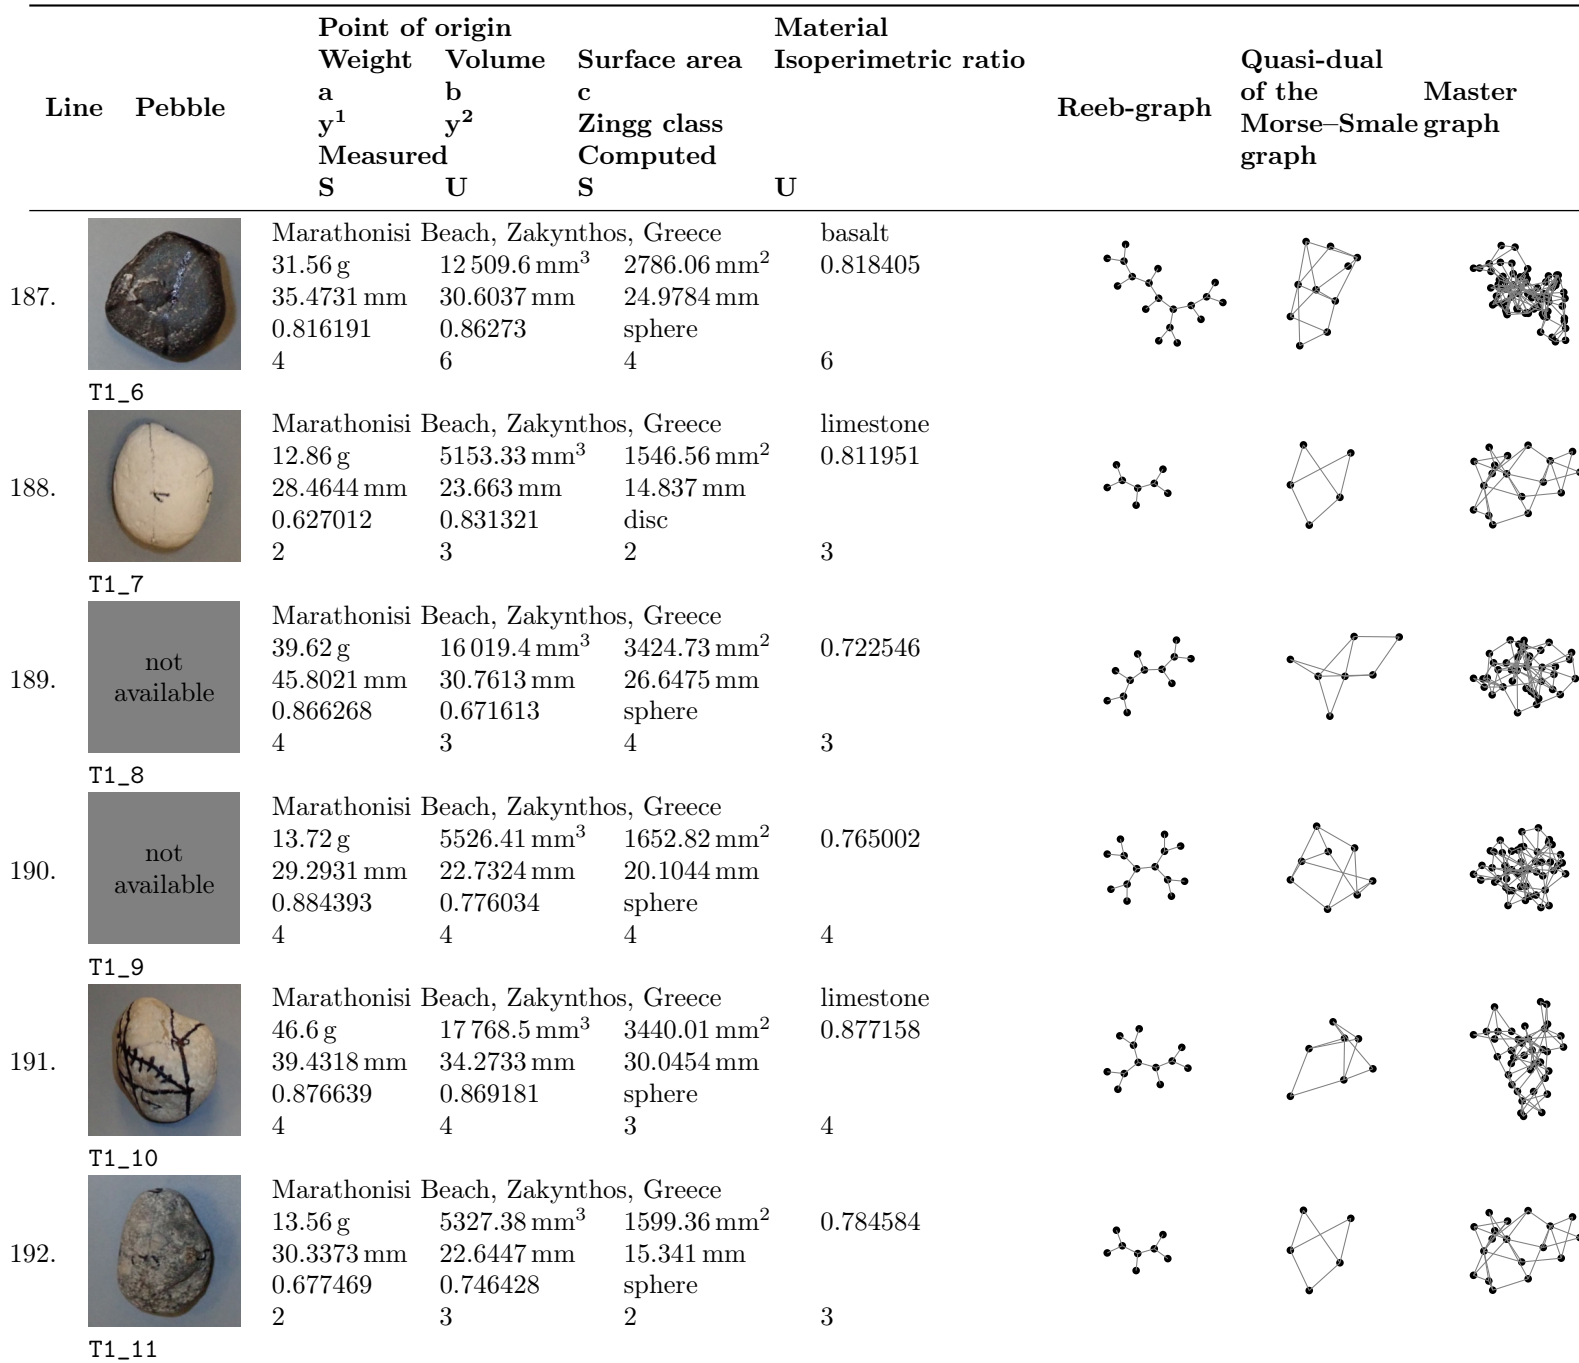   |
| T1_7  |                                                                                     |                                                                                |                                                         |                                                      |                                      |                                                                                       |                                                                                       |                                                                                       |
| 189.  | 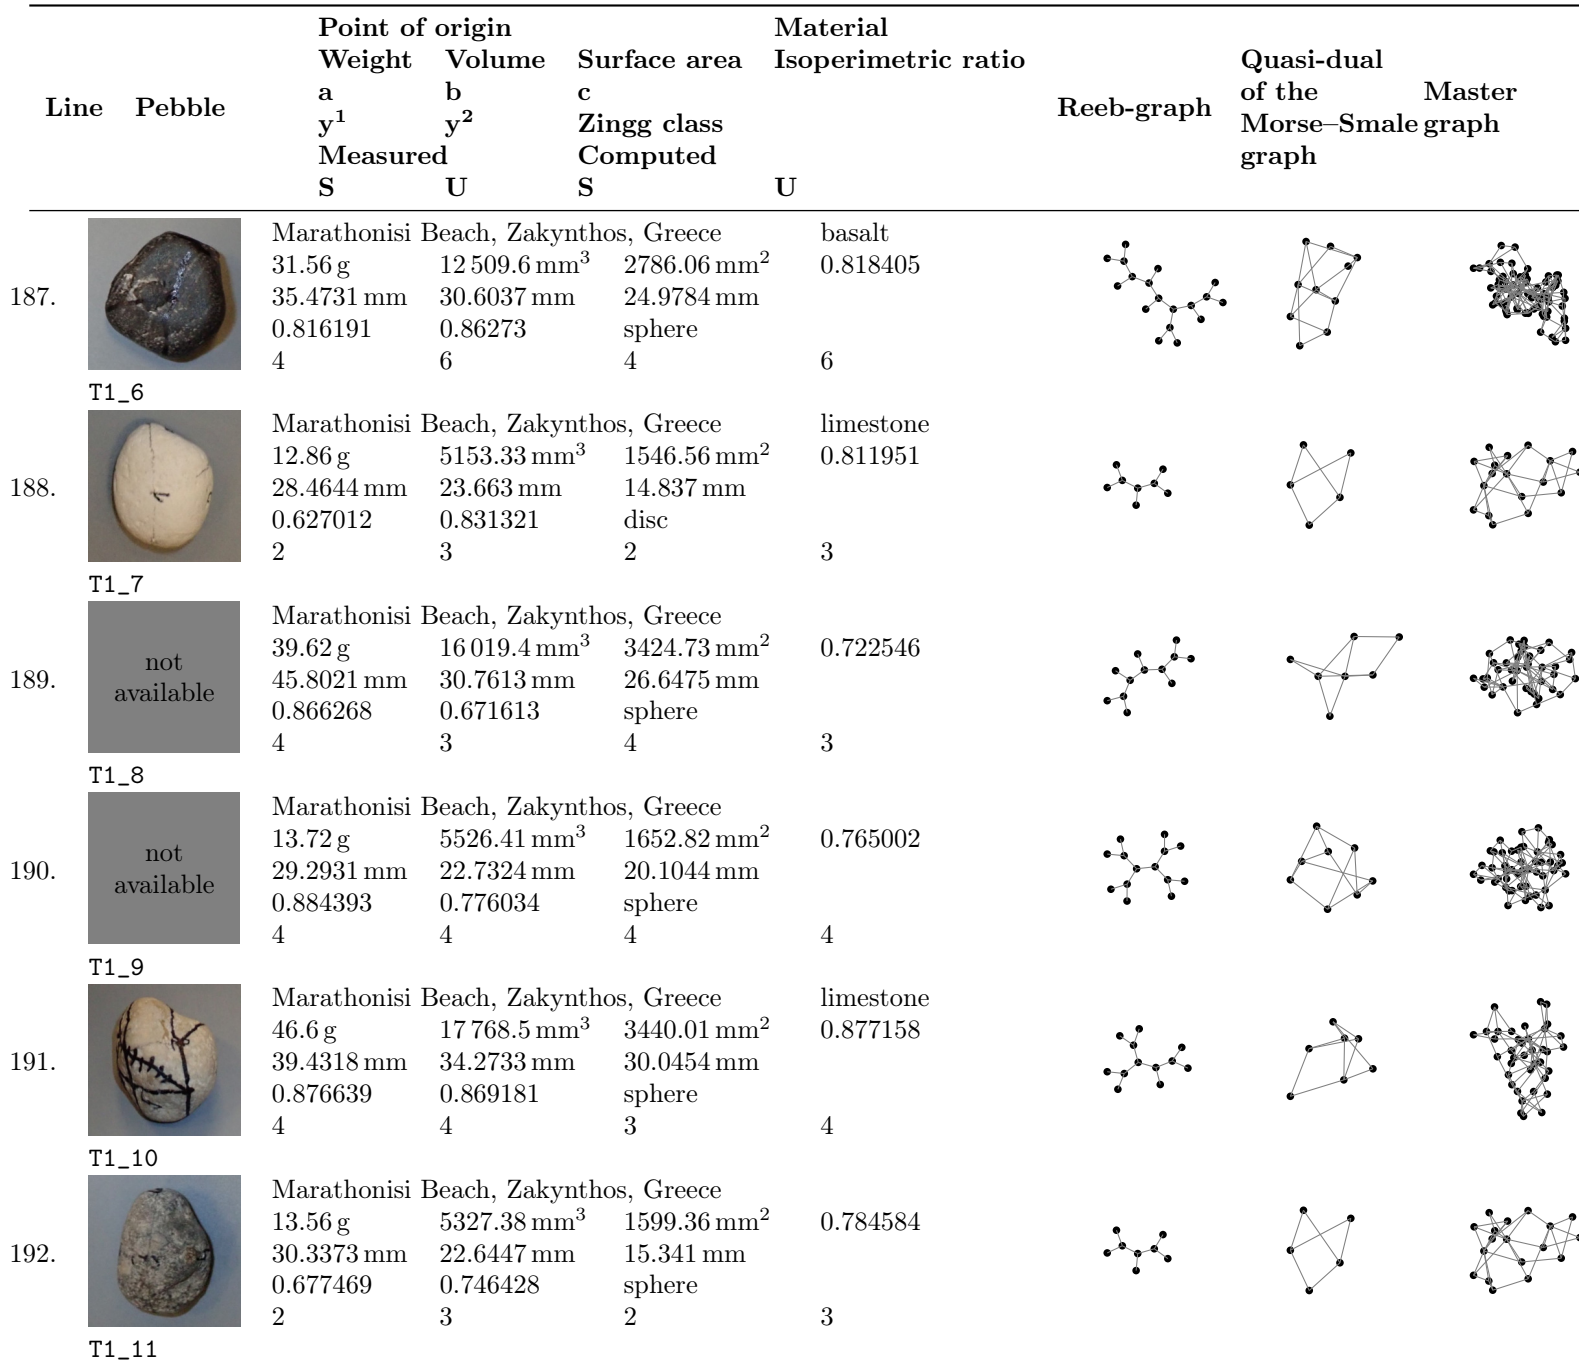   | Marathonisi Beach, Zakynthos, Greece<br>39.62 g<br>45.8021 mm<br>0.866268<br>4 | 16 019.4 mm <sup>3</sup><br>30.7613 mm<br>0.671613<br>3 | 3424.73 mm <sup>2</sup><br>26.6475 mm<br>sphere<br>4 | 0.722546<br><br>3                    | 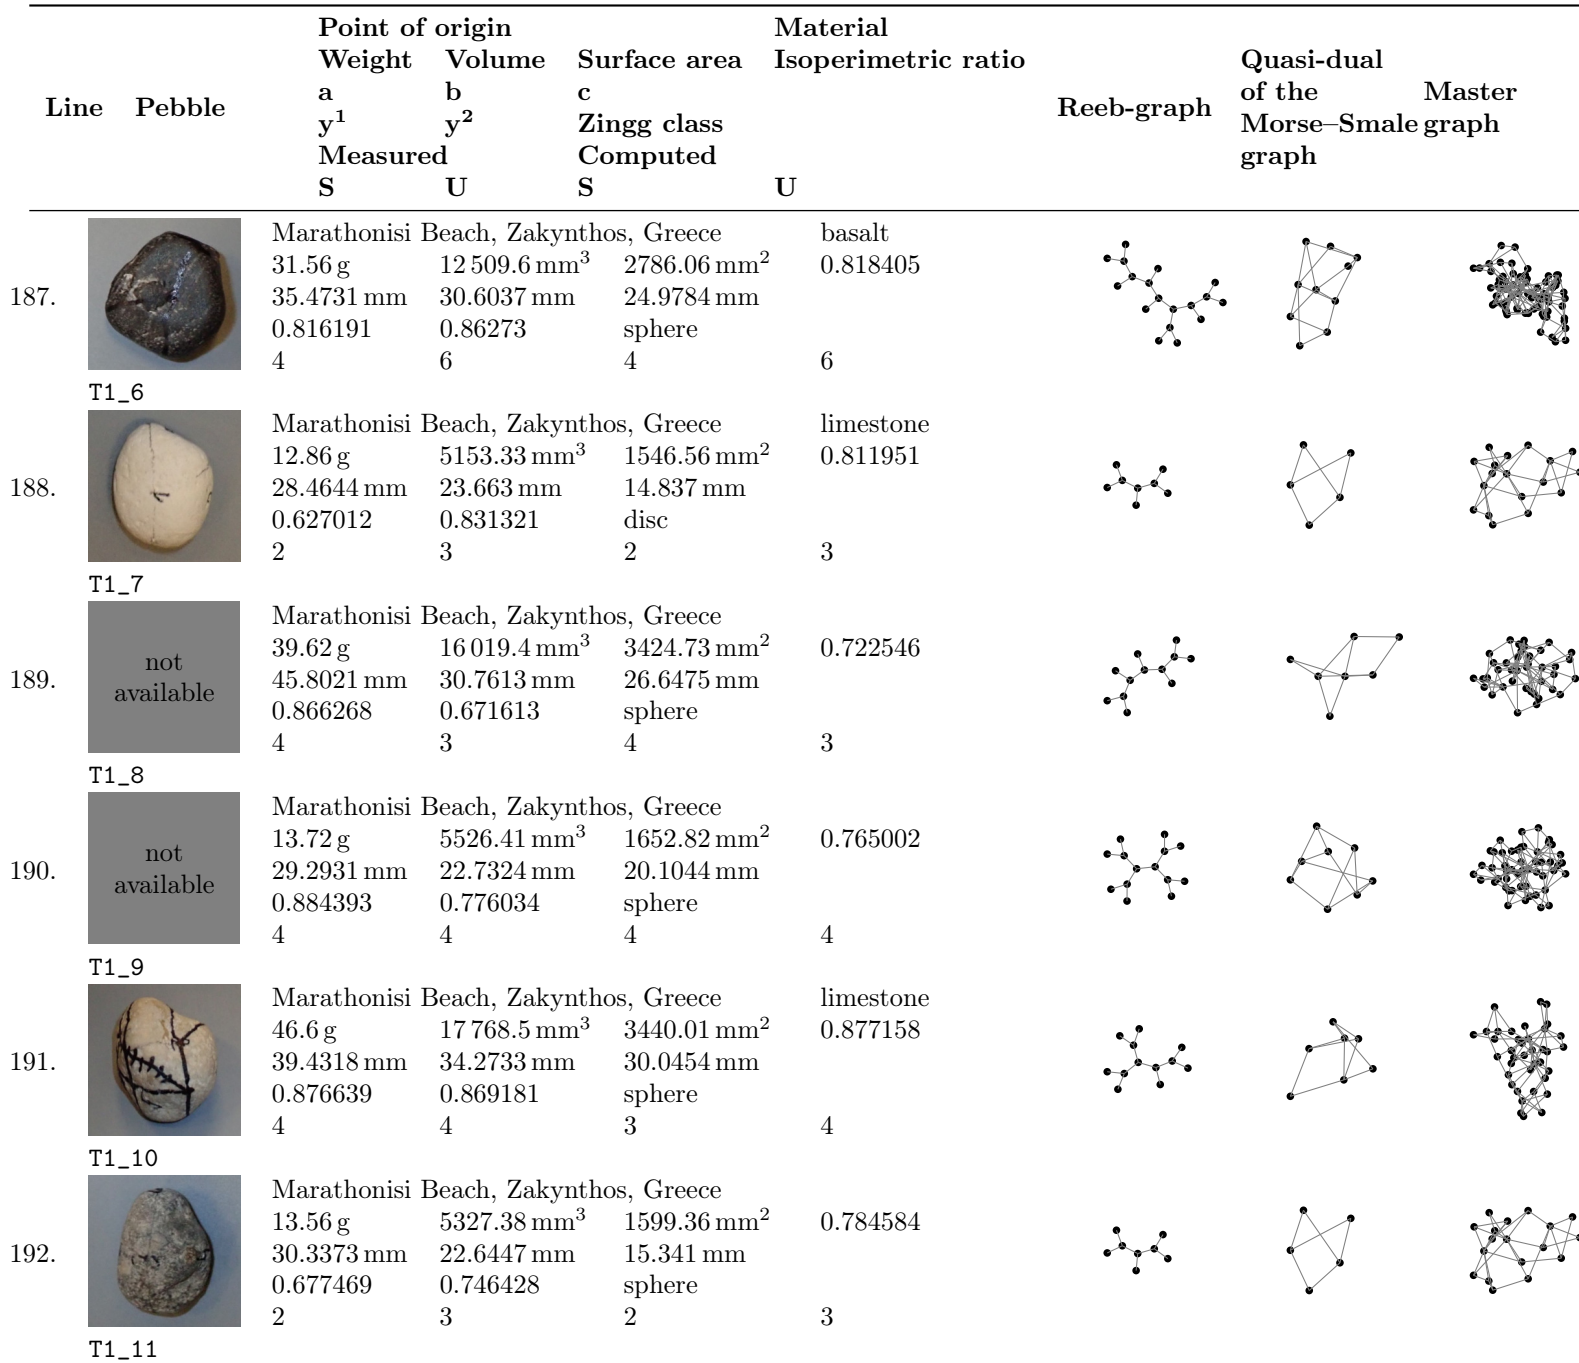   | 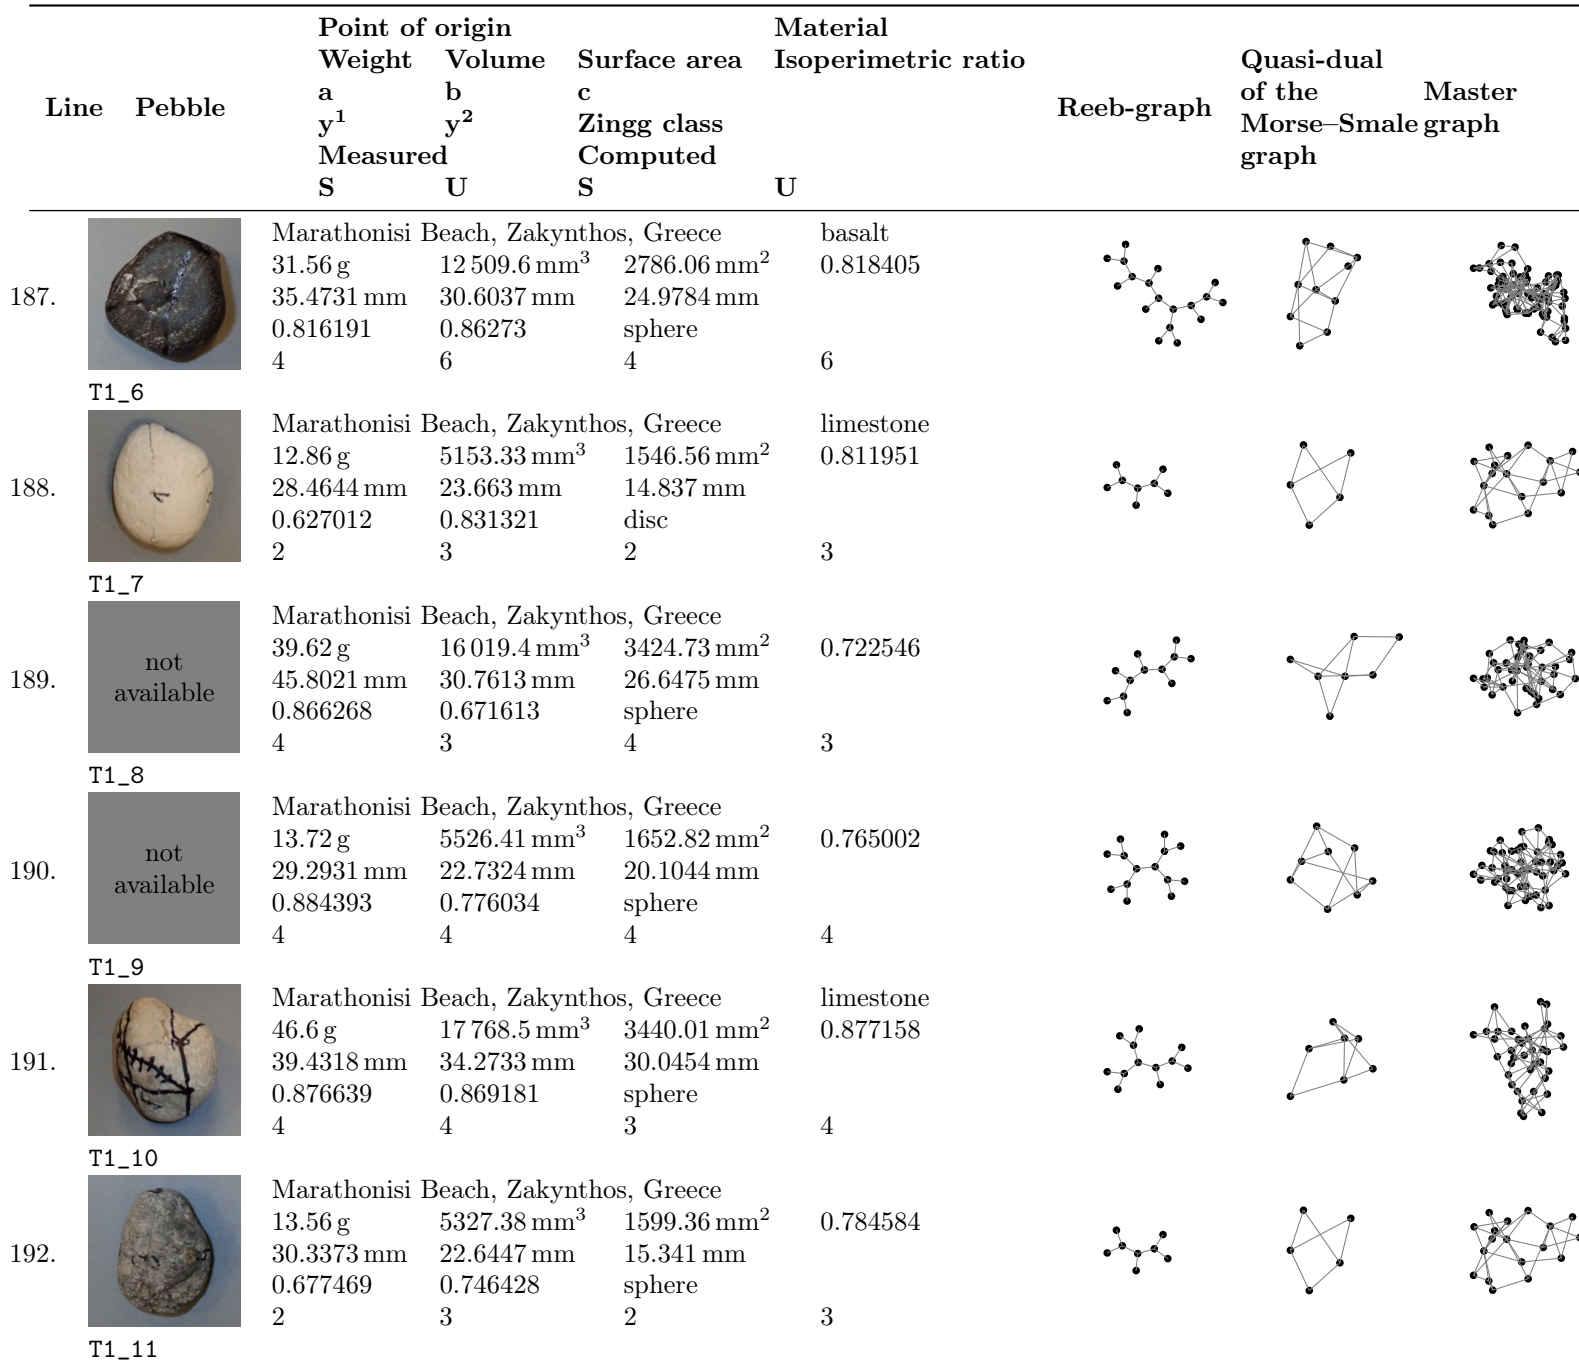   | 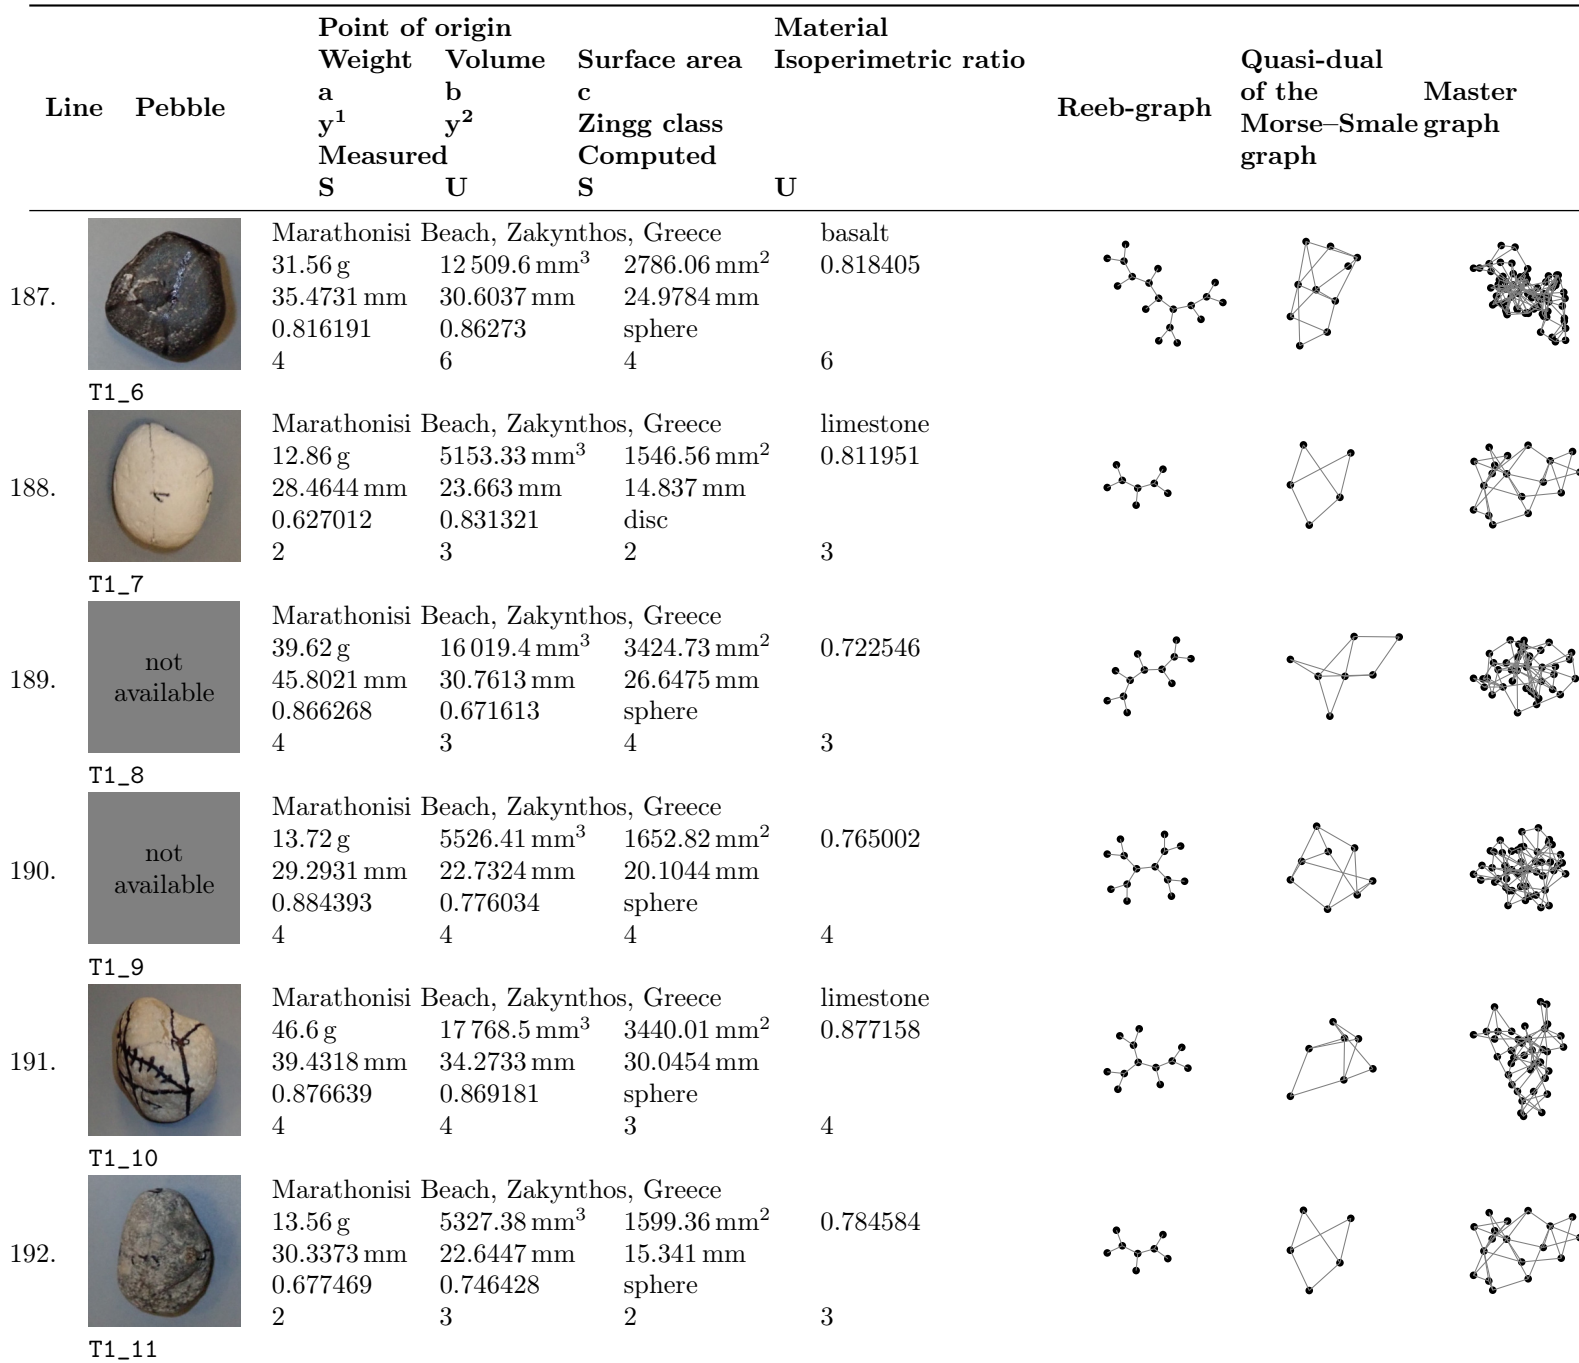   |
| T1_8  |                                                                                     |                                                                                |                                                         |                                                      |                                      |                                                                                       |                                                                                       |                                                                                       |
| 190.  | 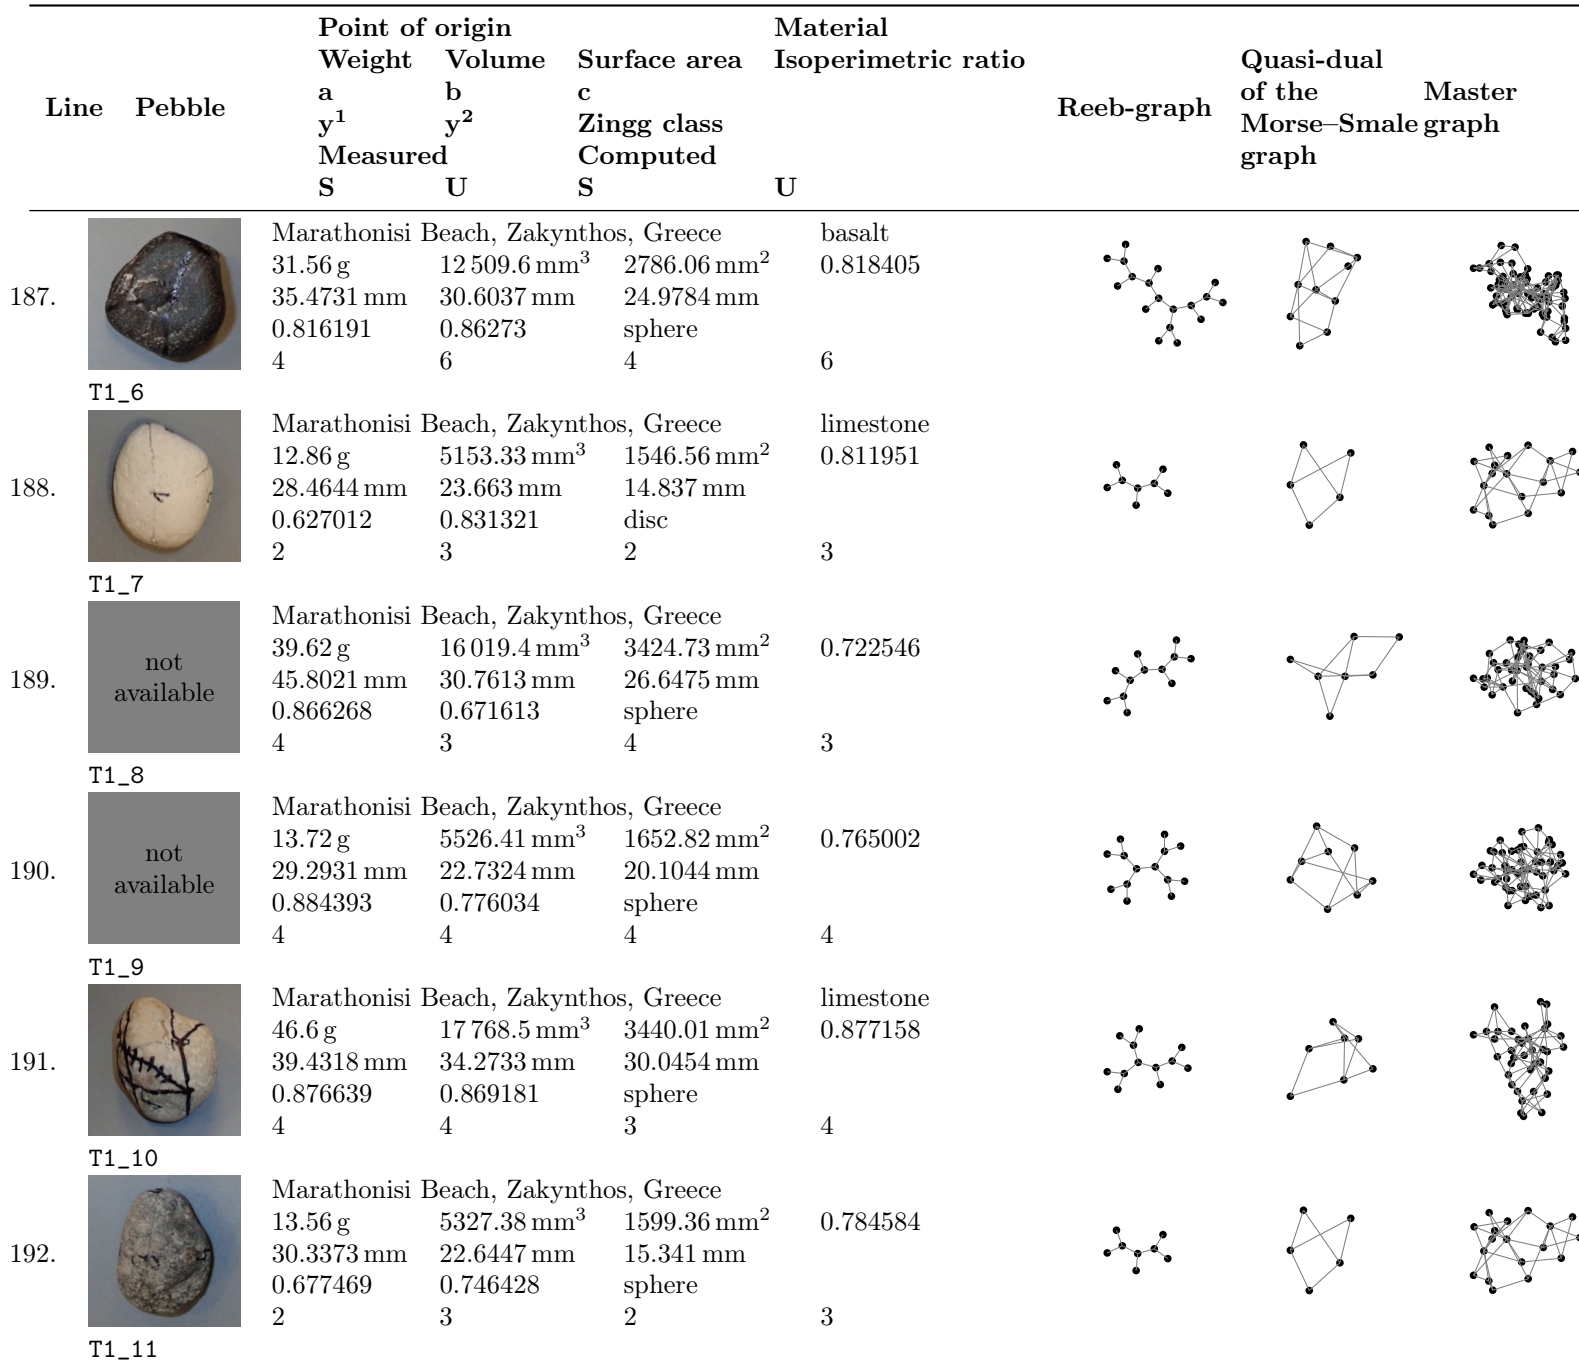  | Marathonisi Beach, Zakynthos, Greece<br>13.72 g<br>29.2931 mm<br>0.884393<br>4 | 5526.41 mm <sup>3</sup><br>22.7324 mm<br>0.776034<br>4  | 1652.82 mm <sup>2</sup><br>20.1044 mm<br>sphere<br>4 | 0.765002<br><br>4                    | 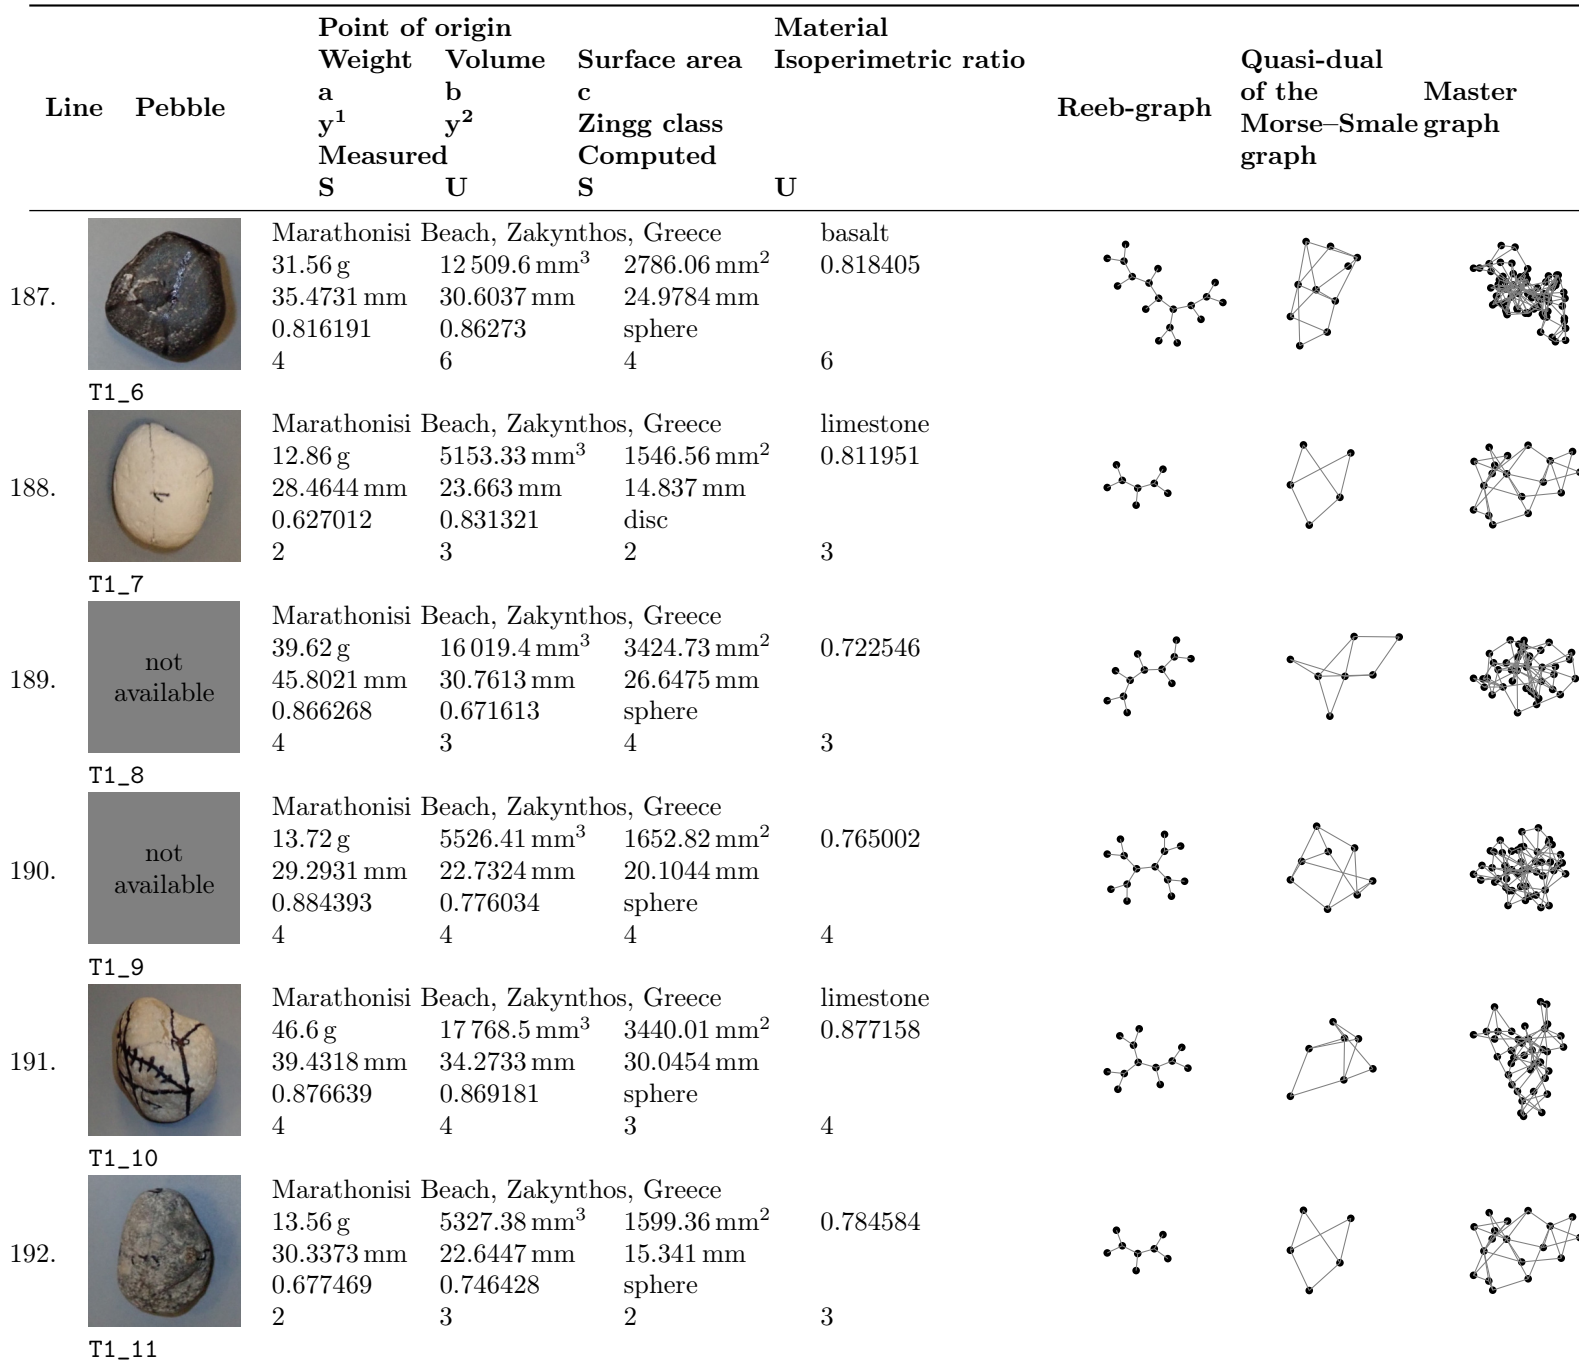  | 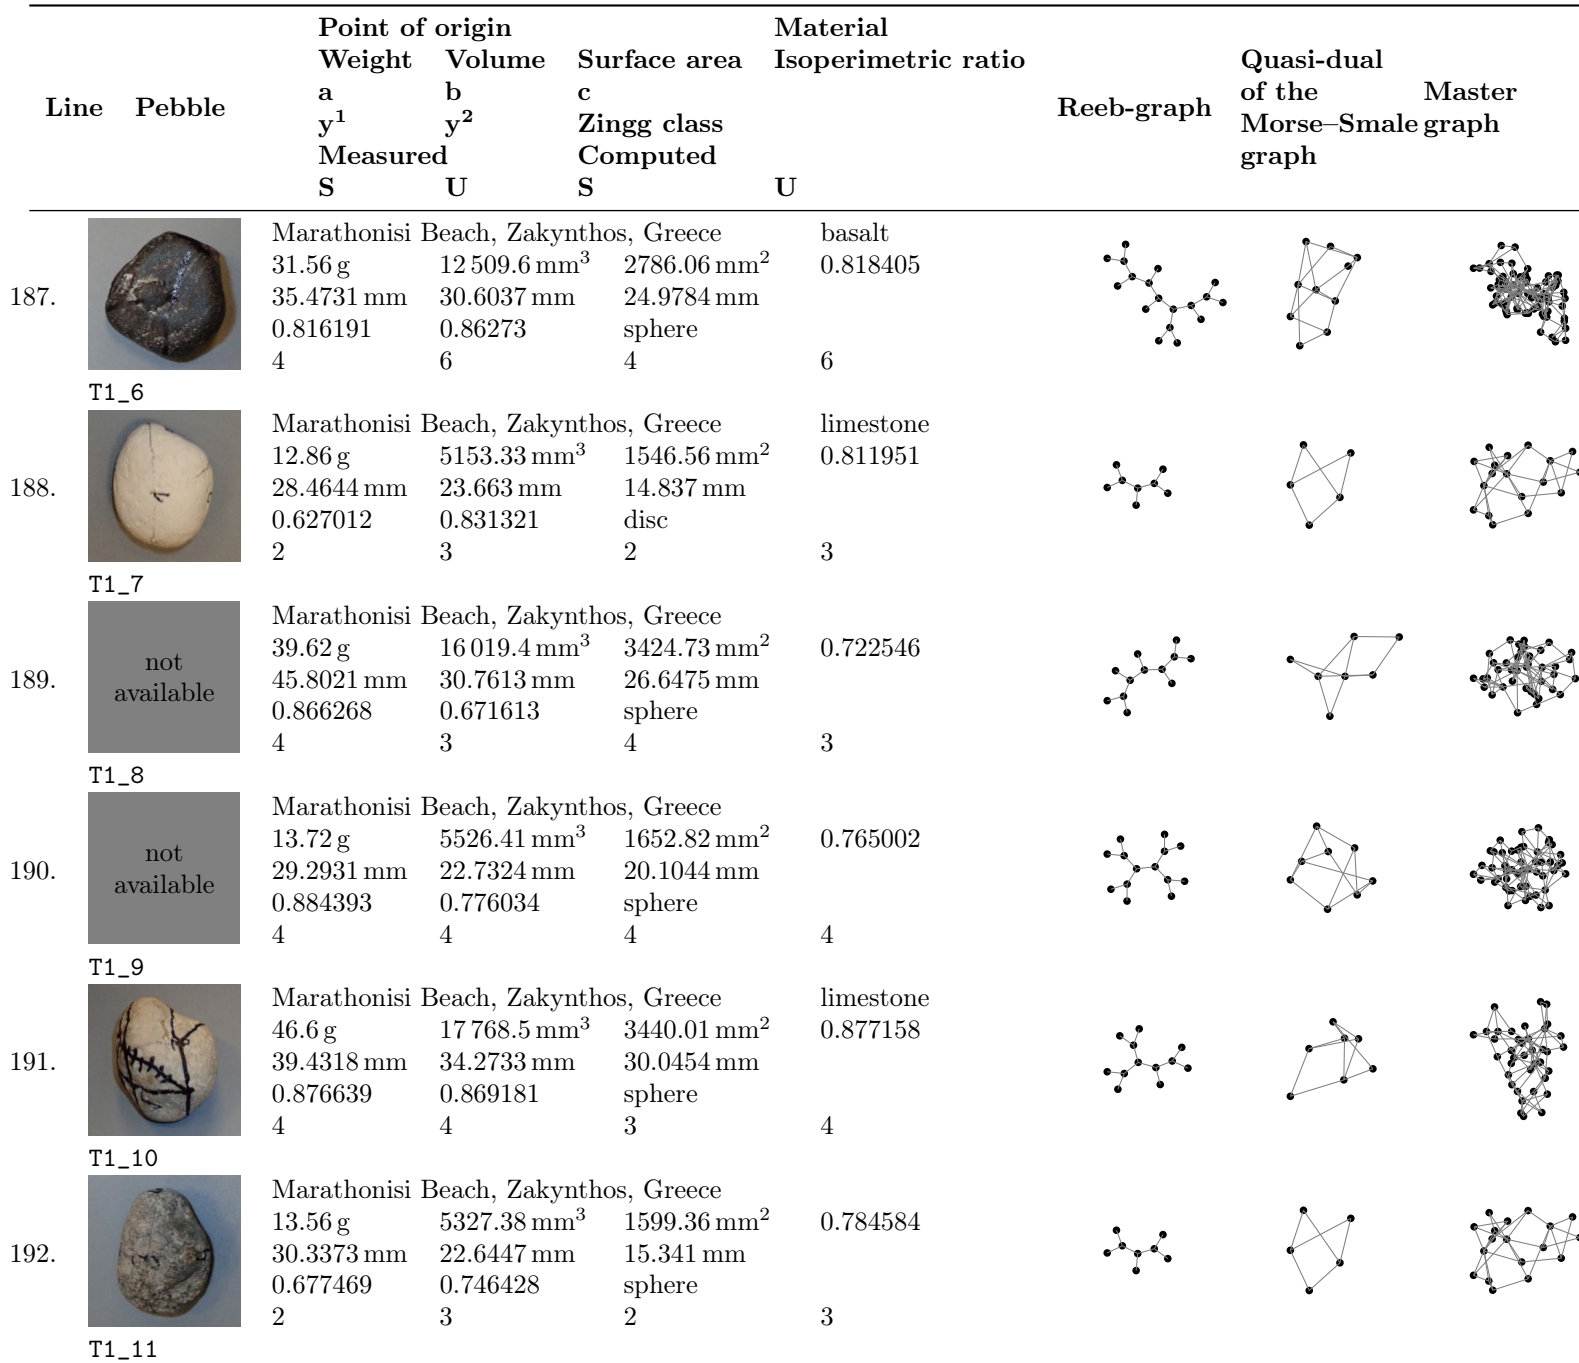  | 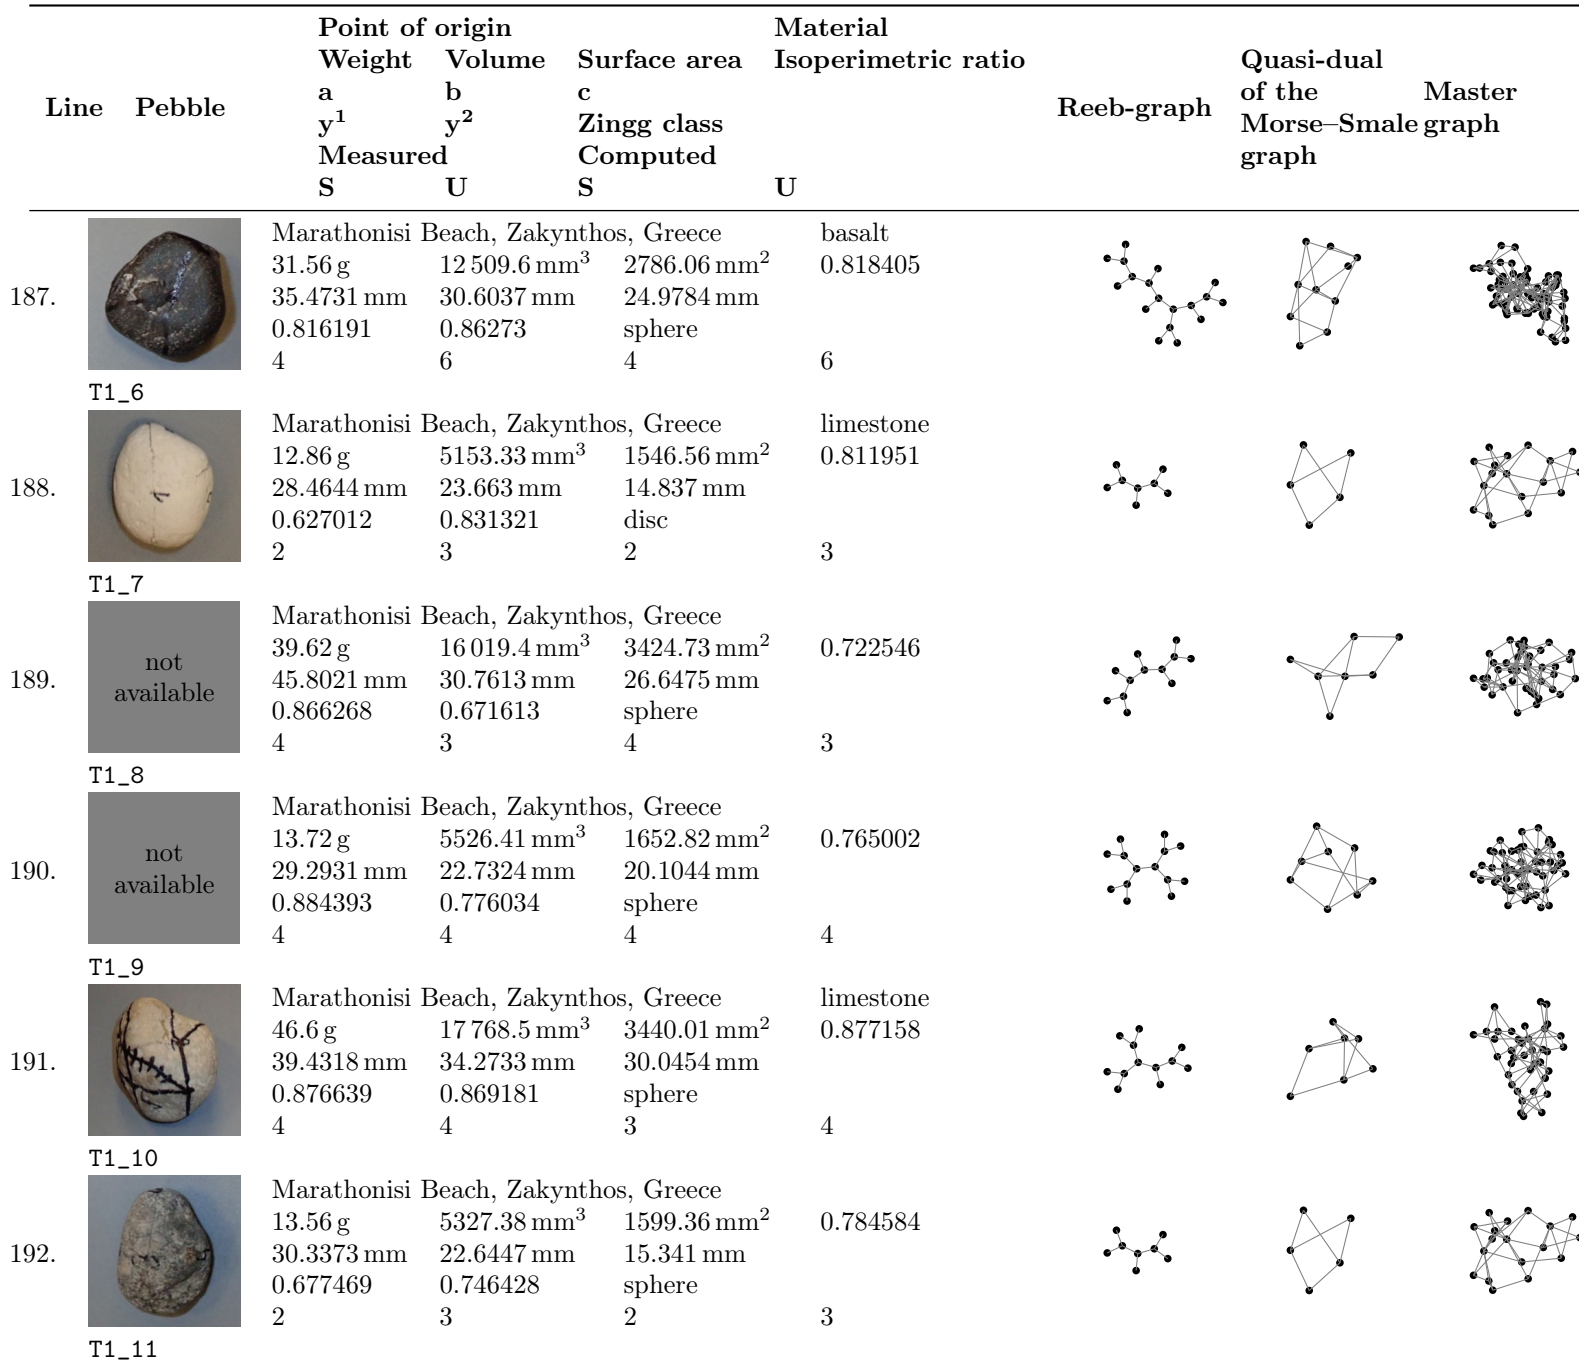  |
| T1_9  |                                                                                     |                                                                                |                                                         |                                                      |                                      |                                                                                       |                                                                                       |                                                                                       |
| 191.  | 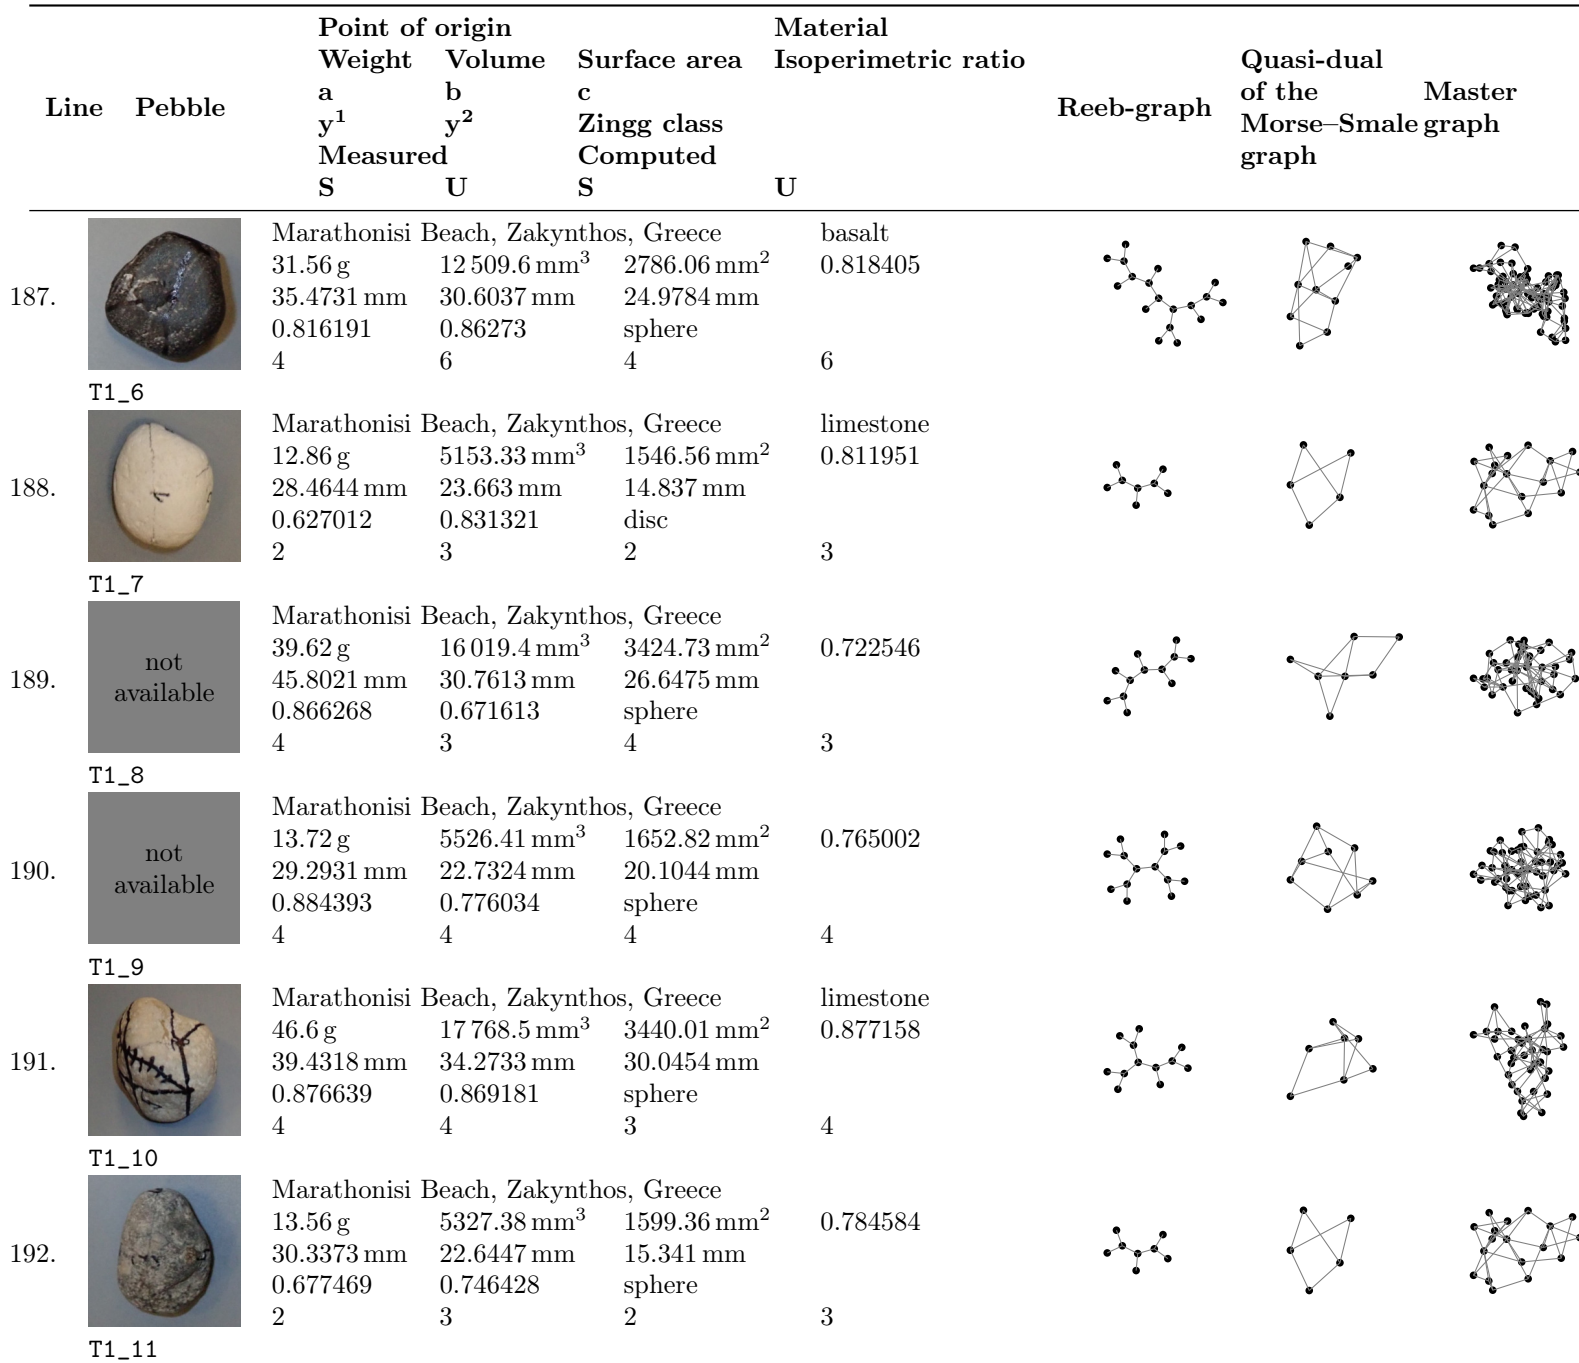 | Marathonisi Beach, Zakynthos, Greece<br>46.6 g<br>39.4318 mm<br>0.876639<br>4  | 17 768.5 mm <sup>3</sup><br>34.2733 mm<br>0.869181<br>4 | 3440.01 mm <sup>2</sup><br>30.0454 mm<br>sphere<br>3 | limestone<br>0.877158<br><br>4       | 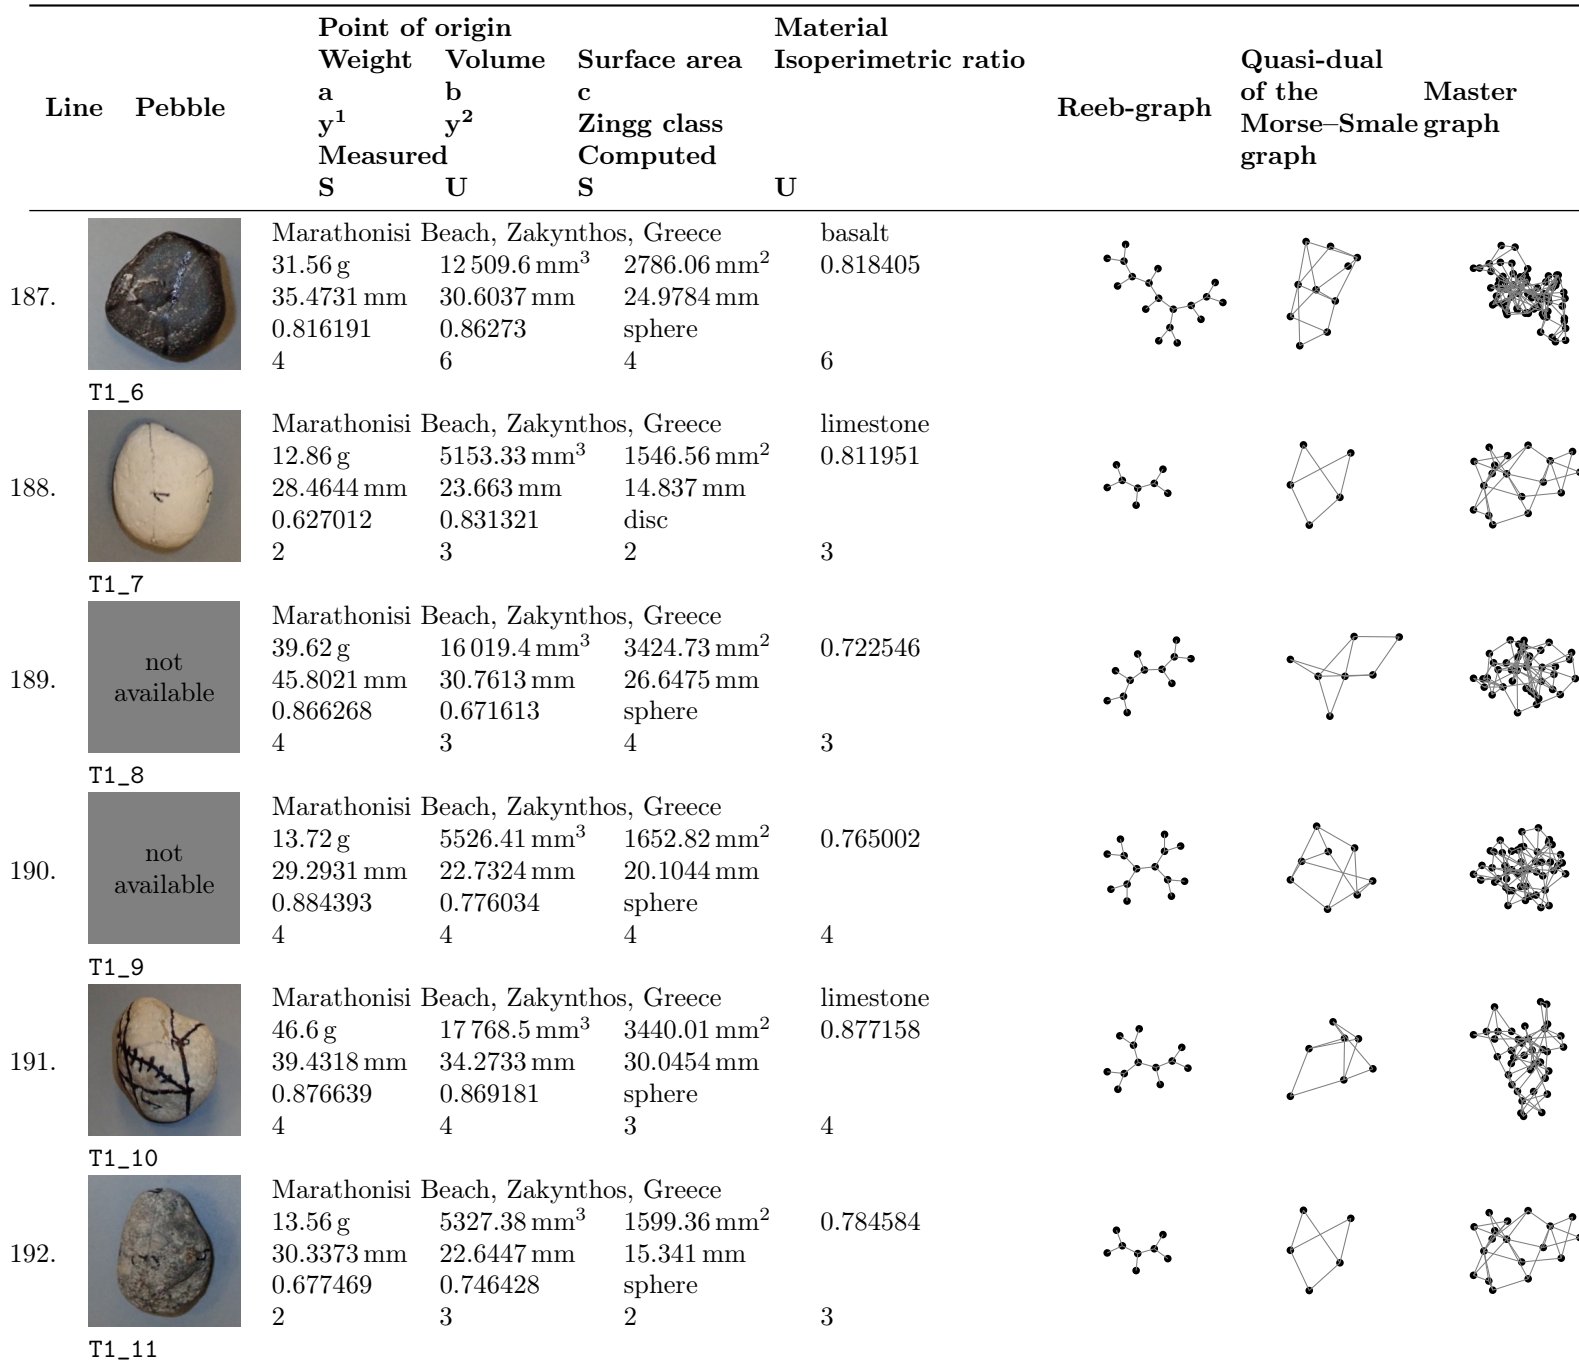 | 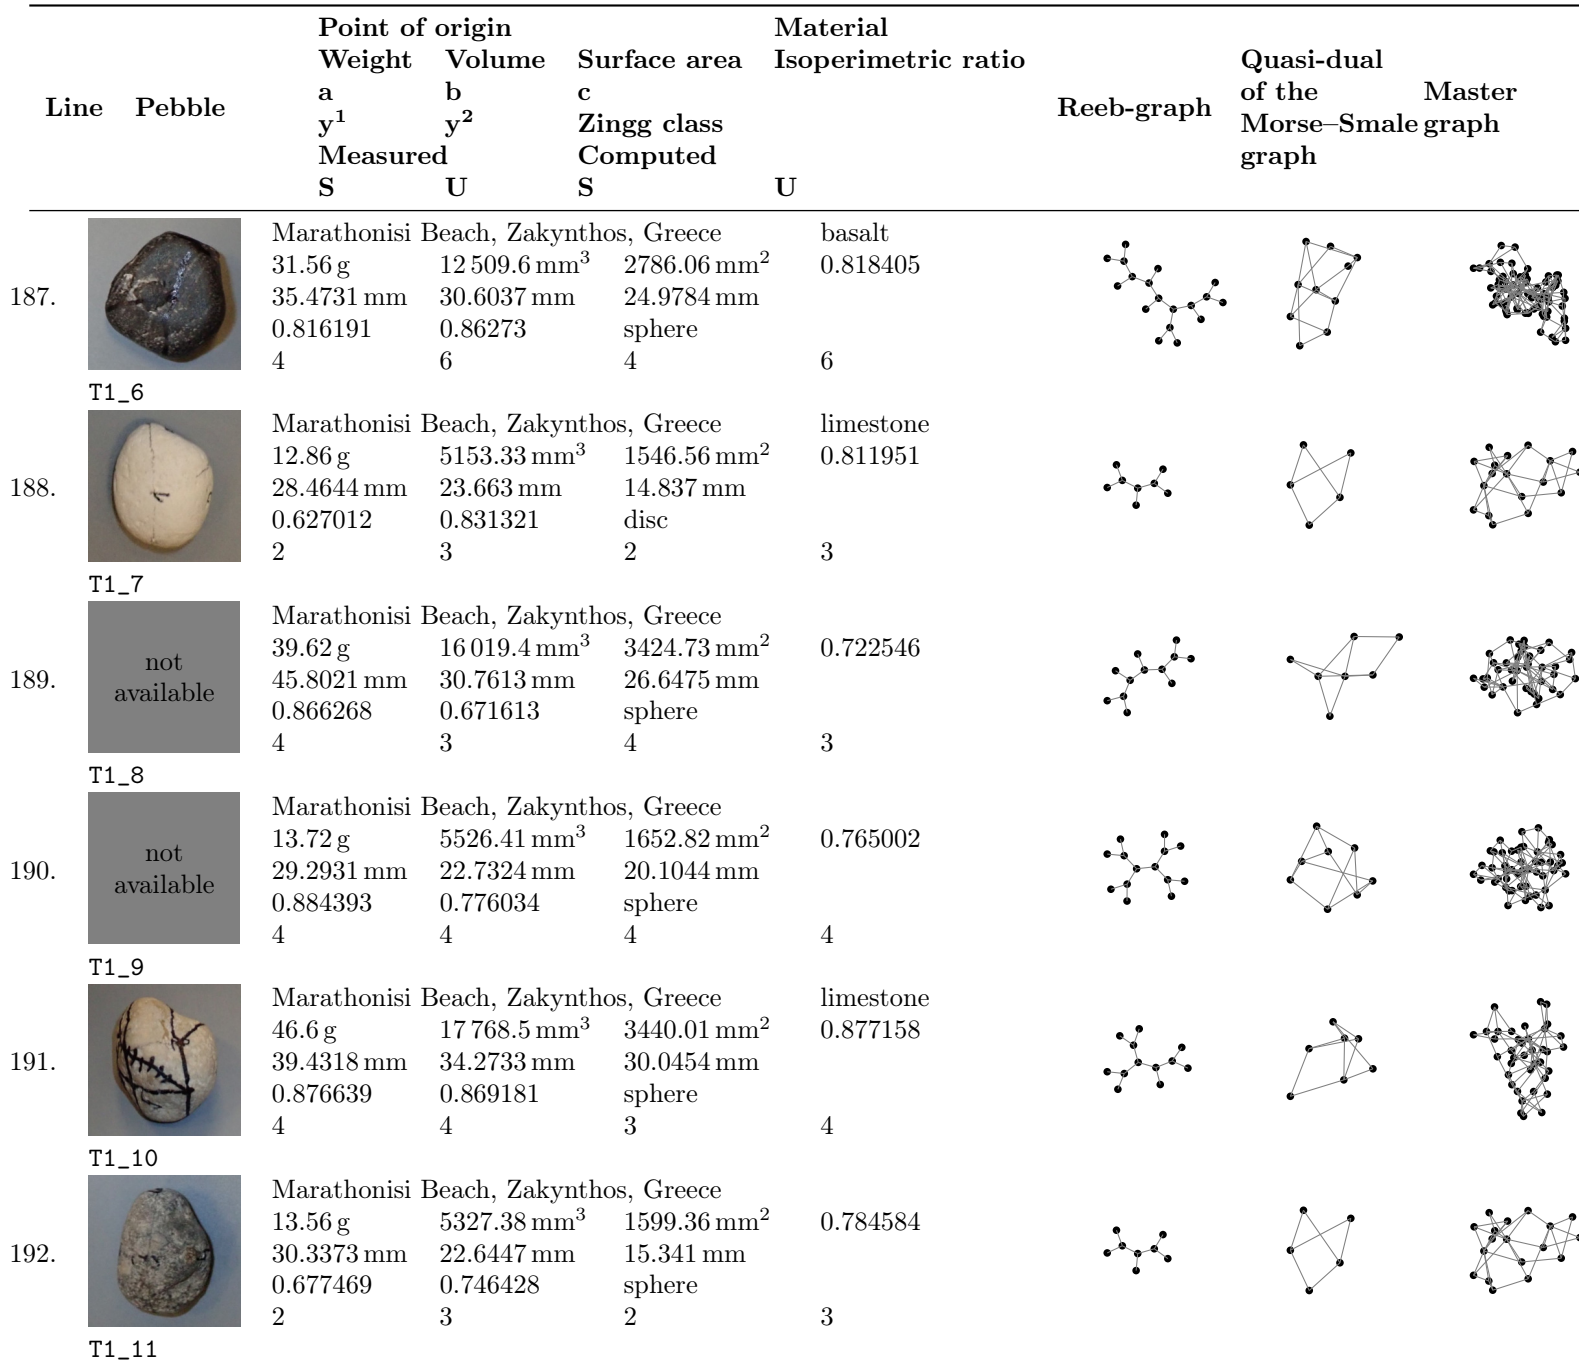 | 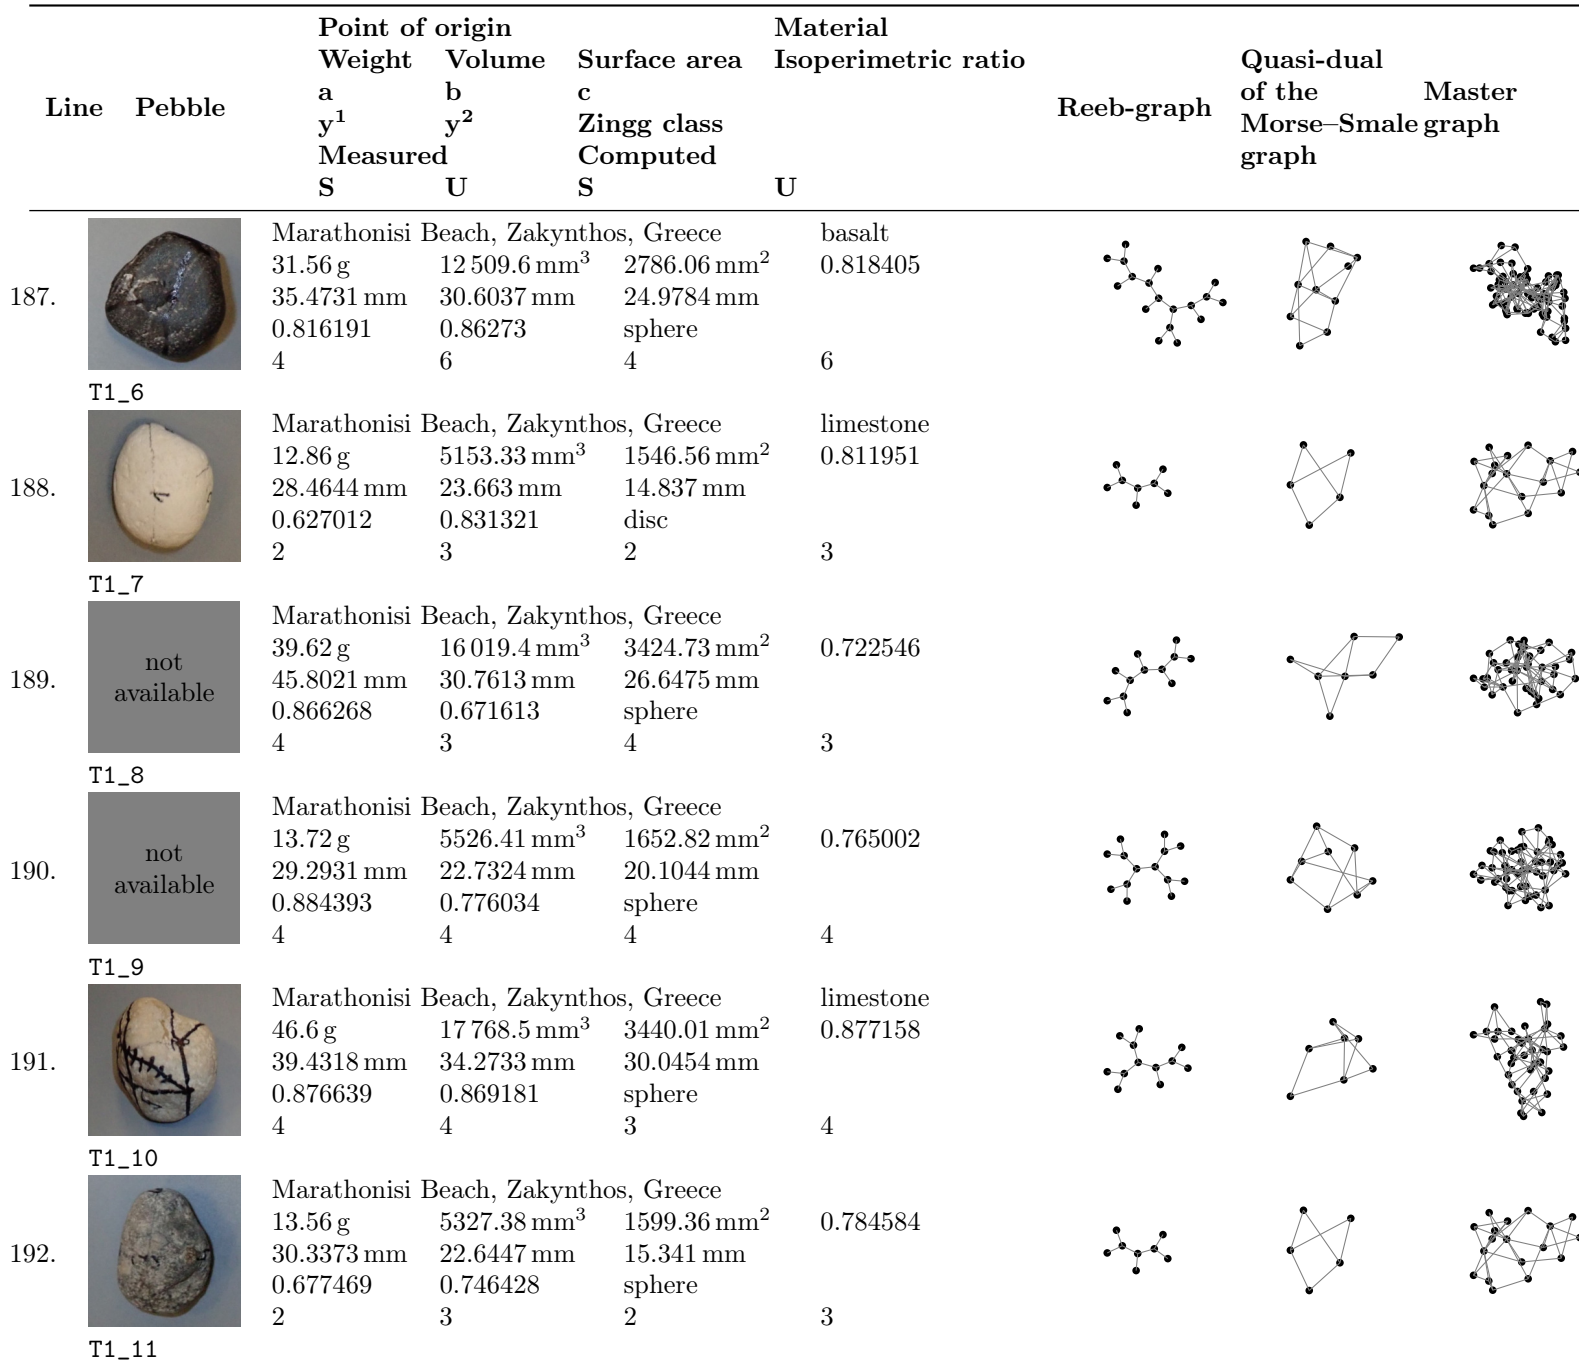 |
| T1_10 |                                                                                     |                                                                                |                                                         |                                                      |                                      |                                                                                       |                                                                                       |                                                                                       |
| 192.  | 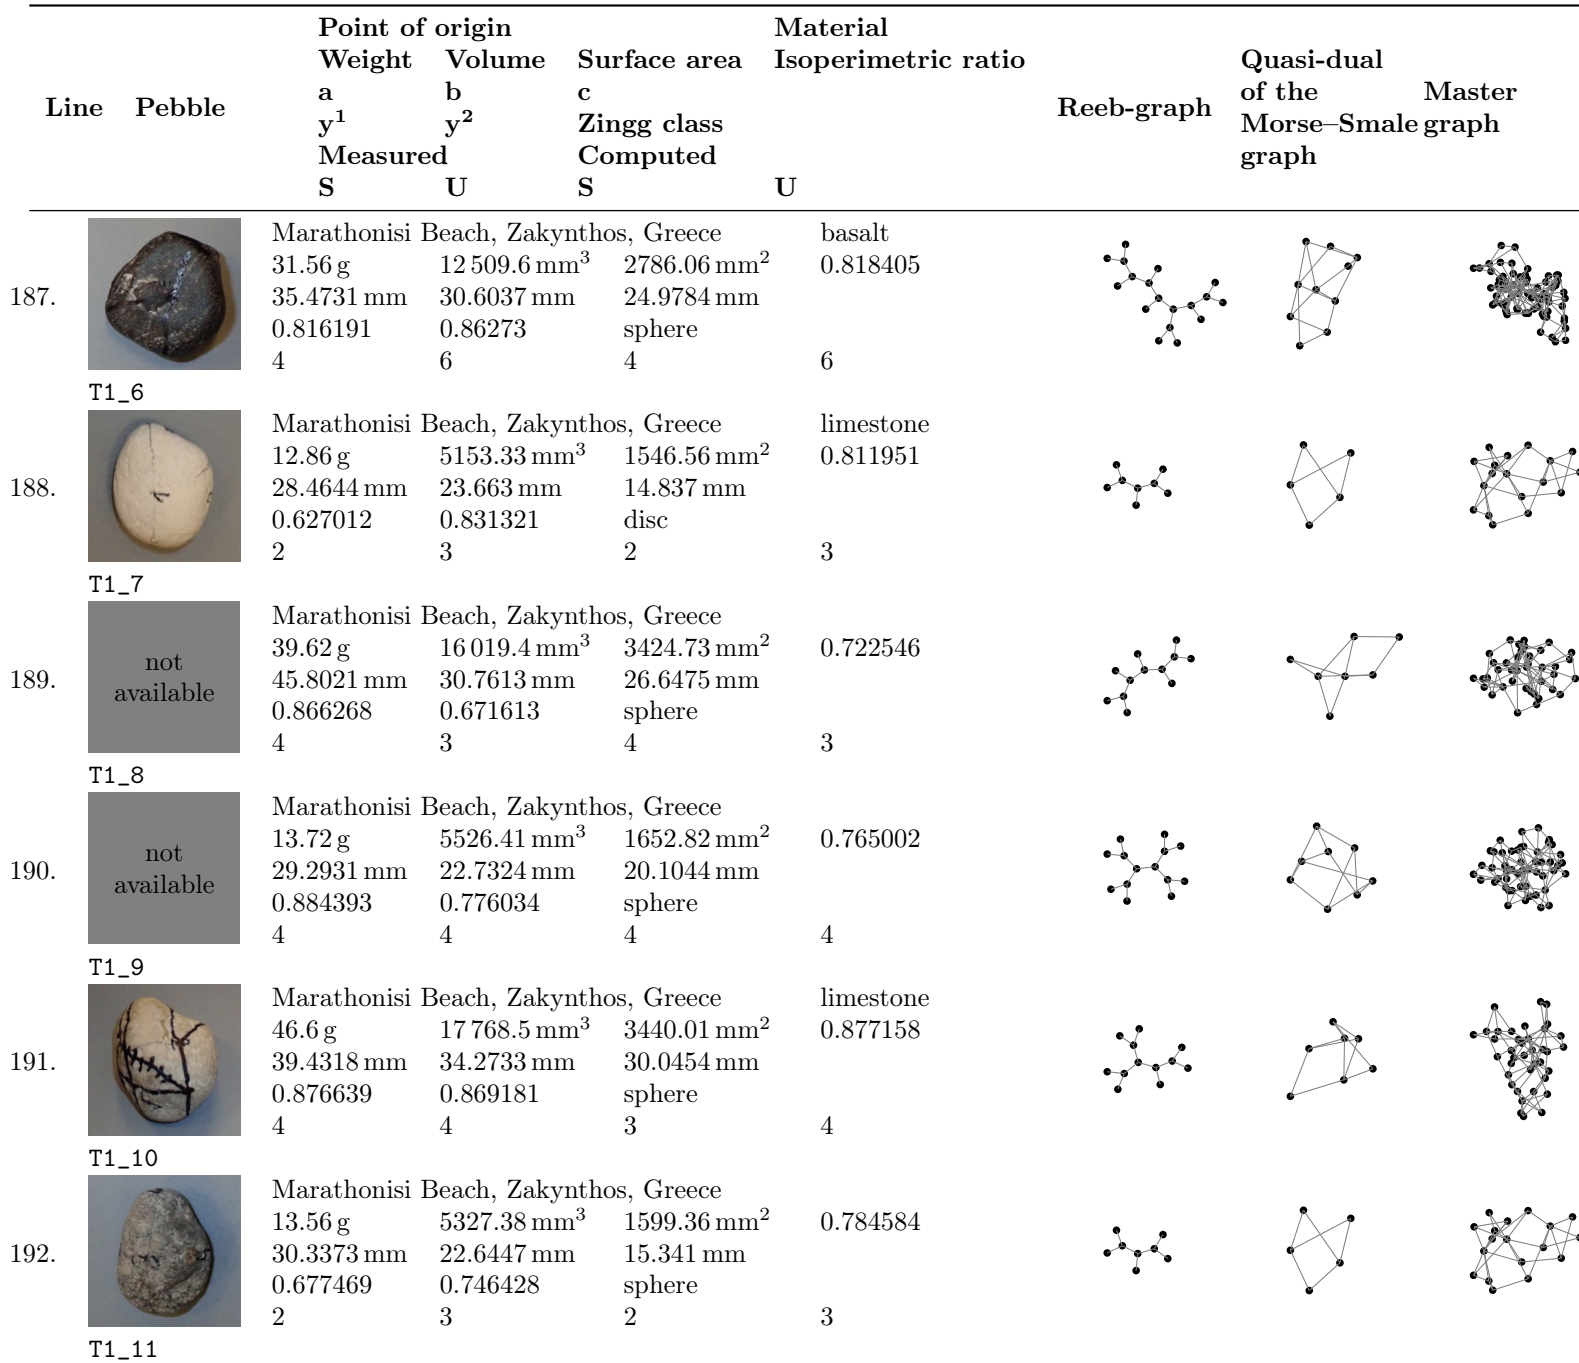 | Marathonisi Beach, Zakynthos, Greece<br>13.56 g<br>30.3373 mm<br>0.677469<br>2 | 5327.38 mm <sup>3</sup><br>22.6447 mm<br>0.746428<br>3  | 1599.36 mm <sup>2</sup><br>15.341 mm<br>sphere<br>2  | 0.784584<br><br>3                    | 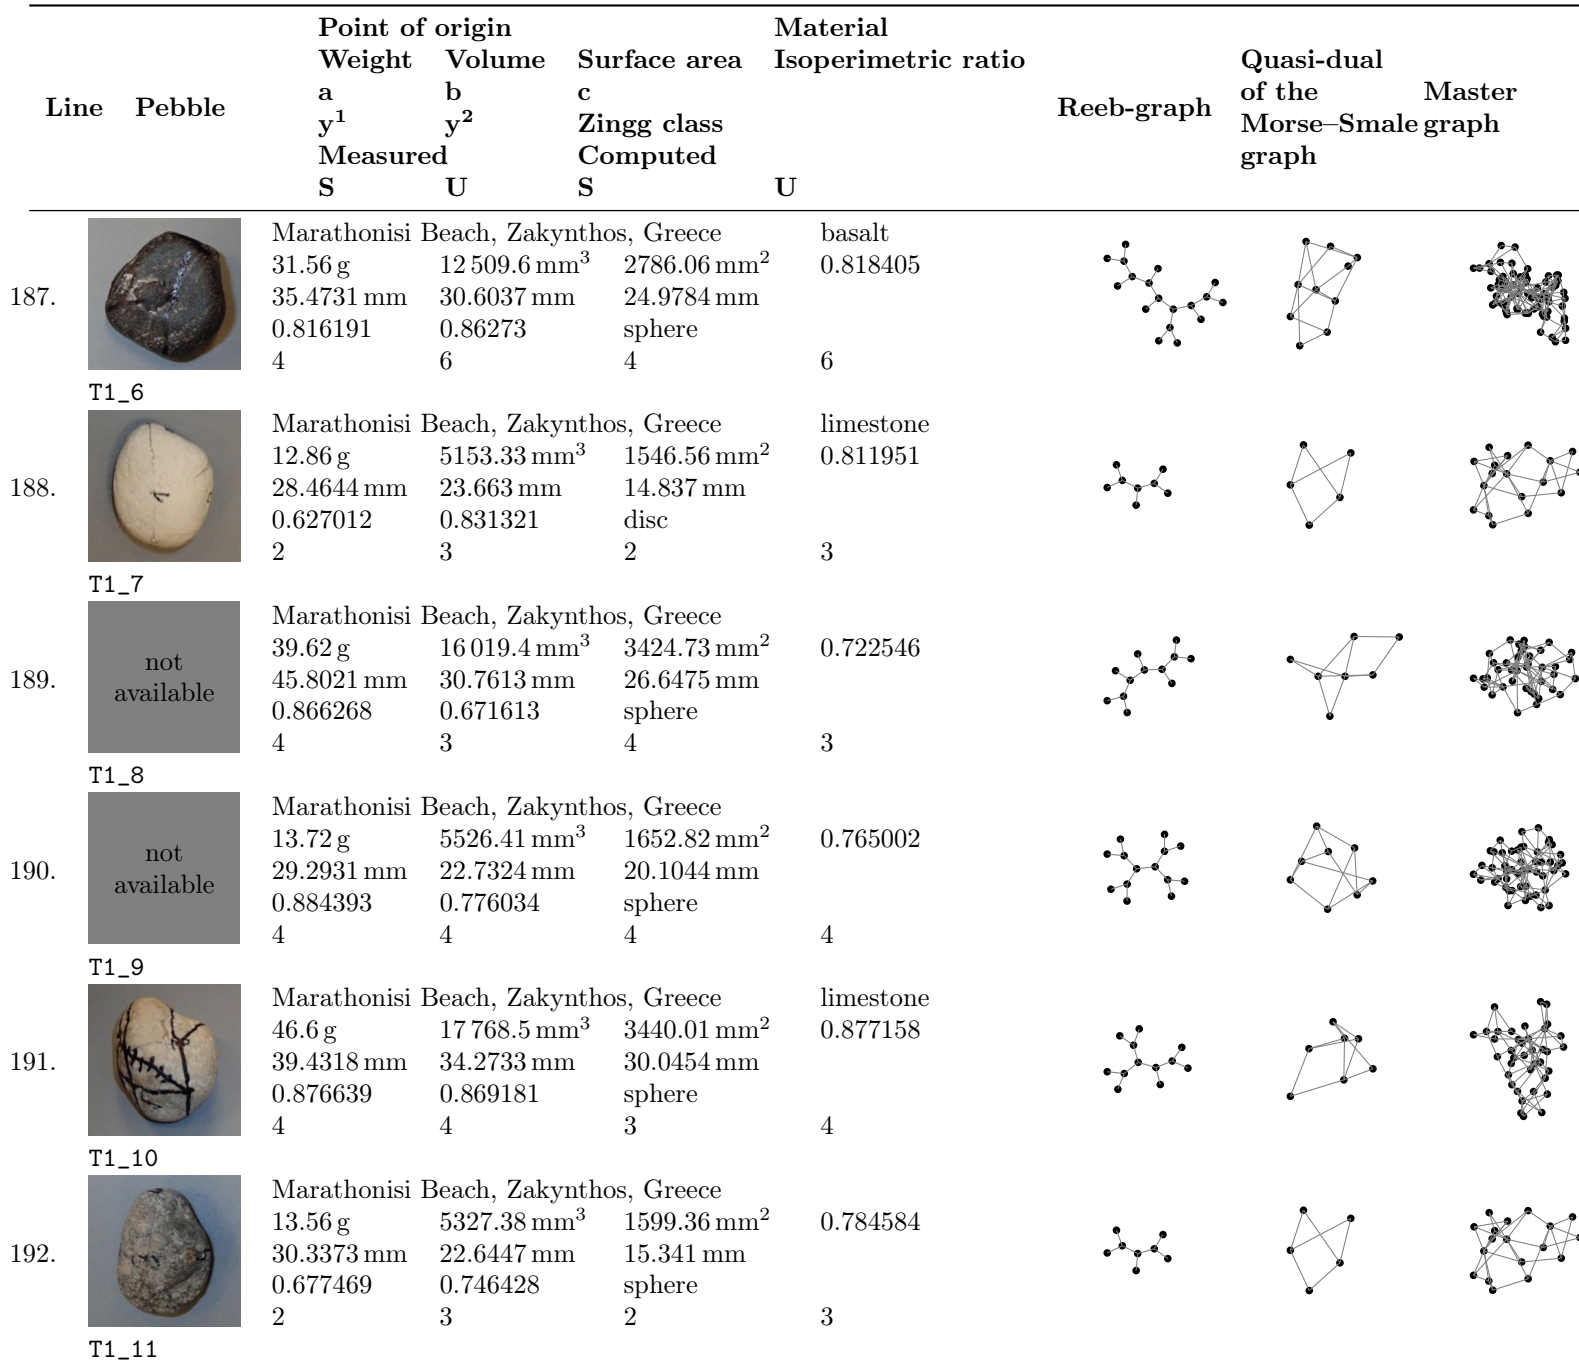 | 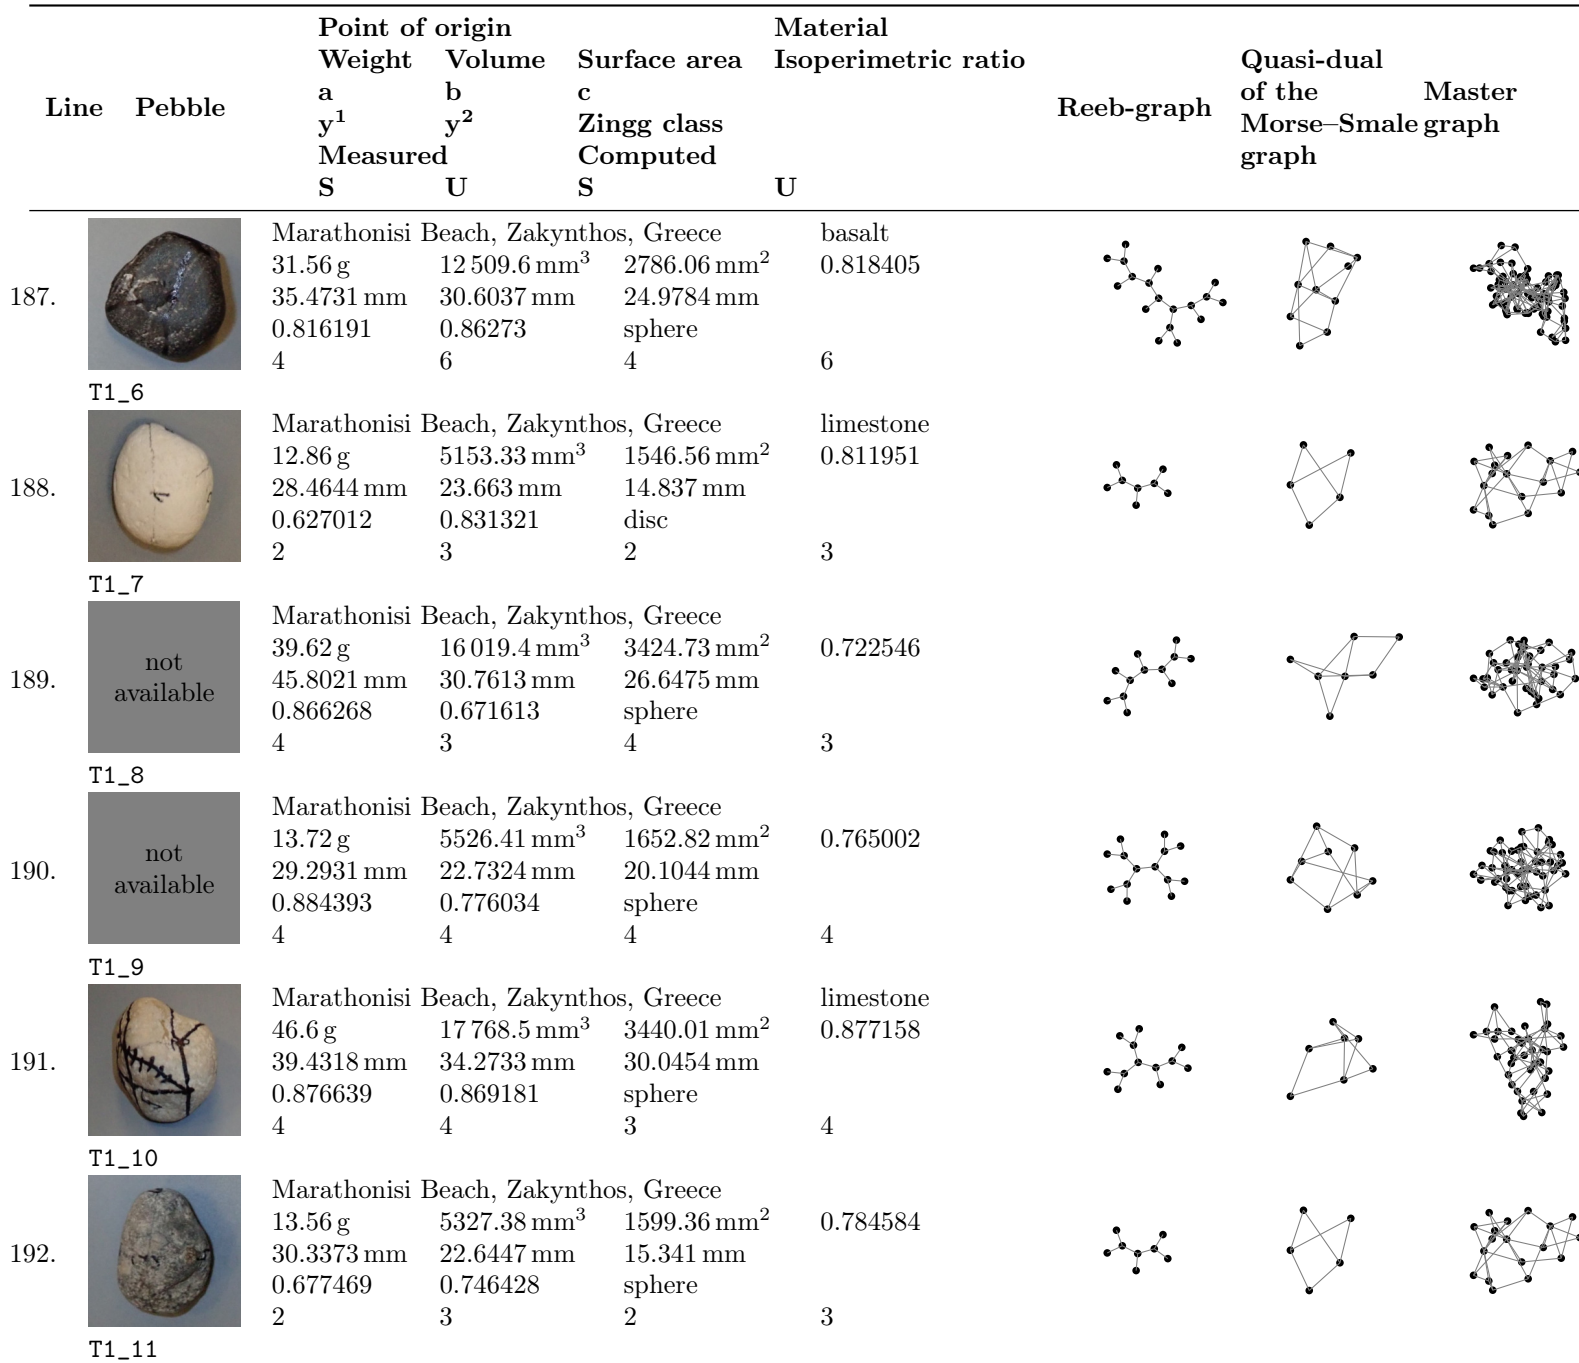 | 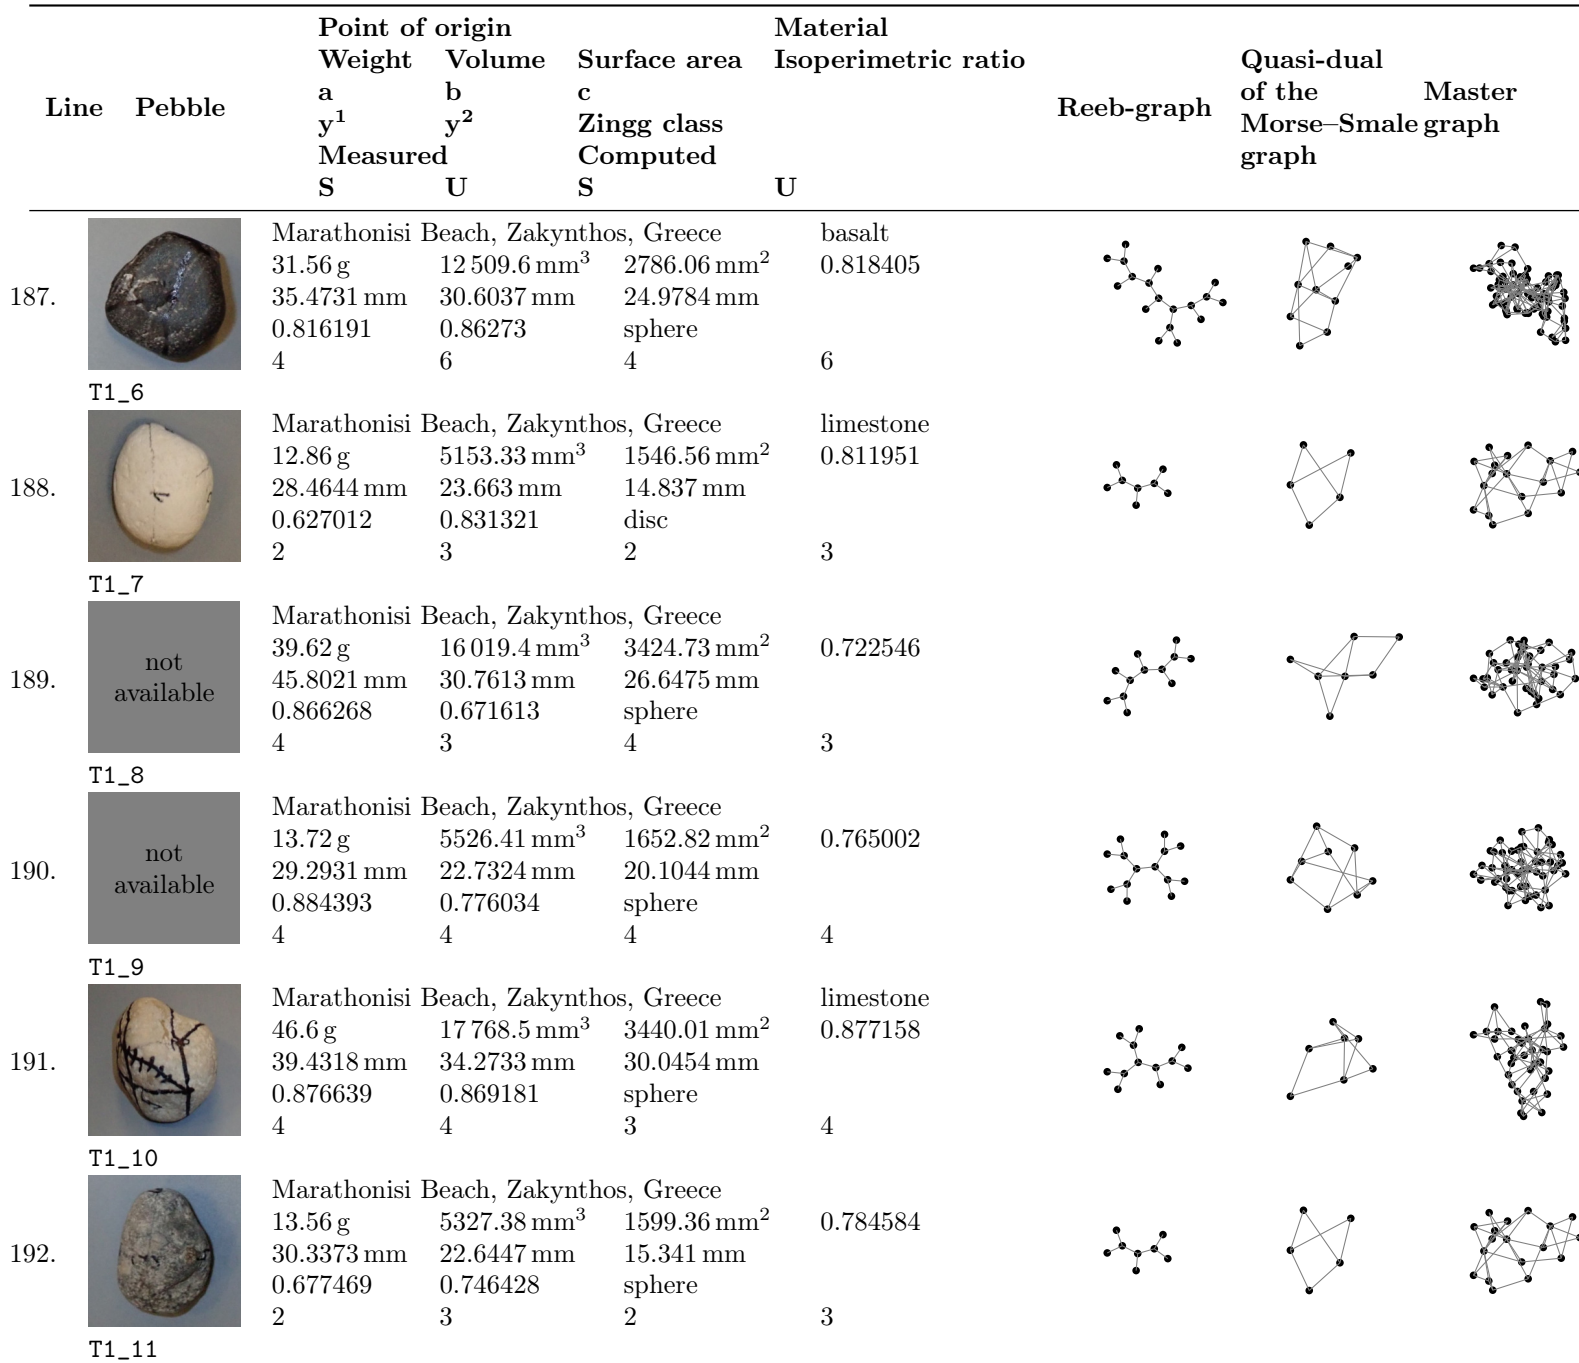 |
| T1_11 |                                                                                     |                                                                                |                                                         |                                                      |                                      |                                                                                       |                                                                                       |                                                                                       |

| Line | Pebble                                                                              | Point of origin                                                                |                                                                    |                                                      | Material                       | Isoperimetric ratio | Reeb-graph                                                                            | Quasi-dual<br>of the<br>Morse–Smale<br>graph                                          | Master                                                                                |
|------|-------------------------------------------------------------------------------------|--------------------------------------------------------------------------------|--------------------------------------------------------------------|------------------------------------------------------|--------------------------------|---------------------|---------------------------------------------------------------------------------------|---------------------------------------------------------------------------------------|---------------------------------------------------------------------------------------|
|      |                                                                                     | Weight                                                                         | Volume                                                             | Surface area                                         |                                |                     |                                                                                       |                                                                                       |                                                                                       |
|      |                                                                                     | a                                                                              | b                                                                  | c                                                    |                                |                     |                                                                                       |                                                                                       |                                                                                       |
|      |                                                                                     | y <sup>1</sup><br>Measured<br>S                                                | y <sup>2</sup><br>U                                                | Zingg class<br>Computed<br>S                         |                                |                     |                                                                                       |                                                                                       |                                                                                       |
| 193. | 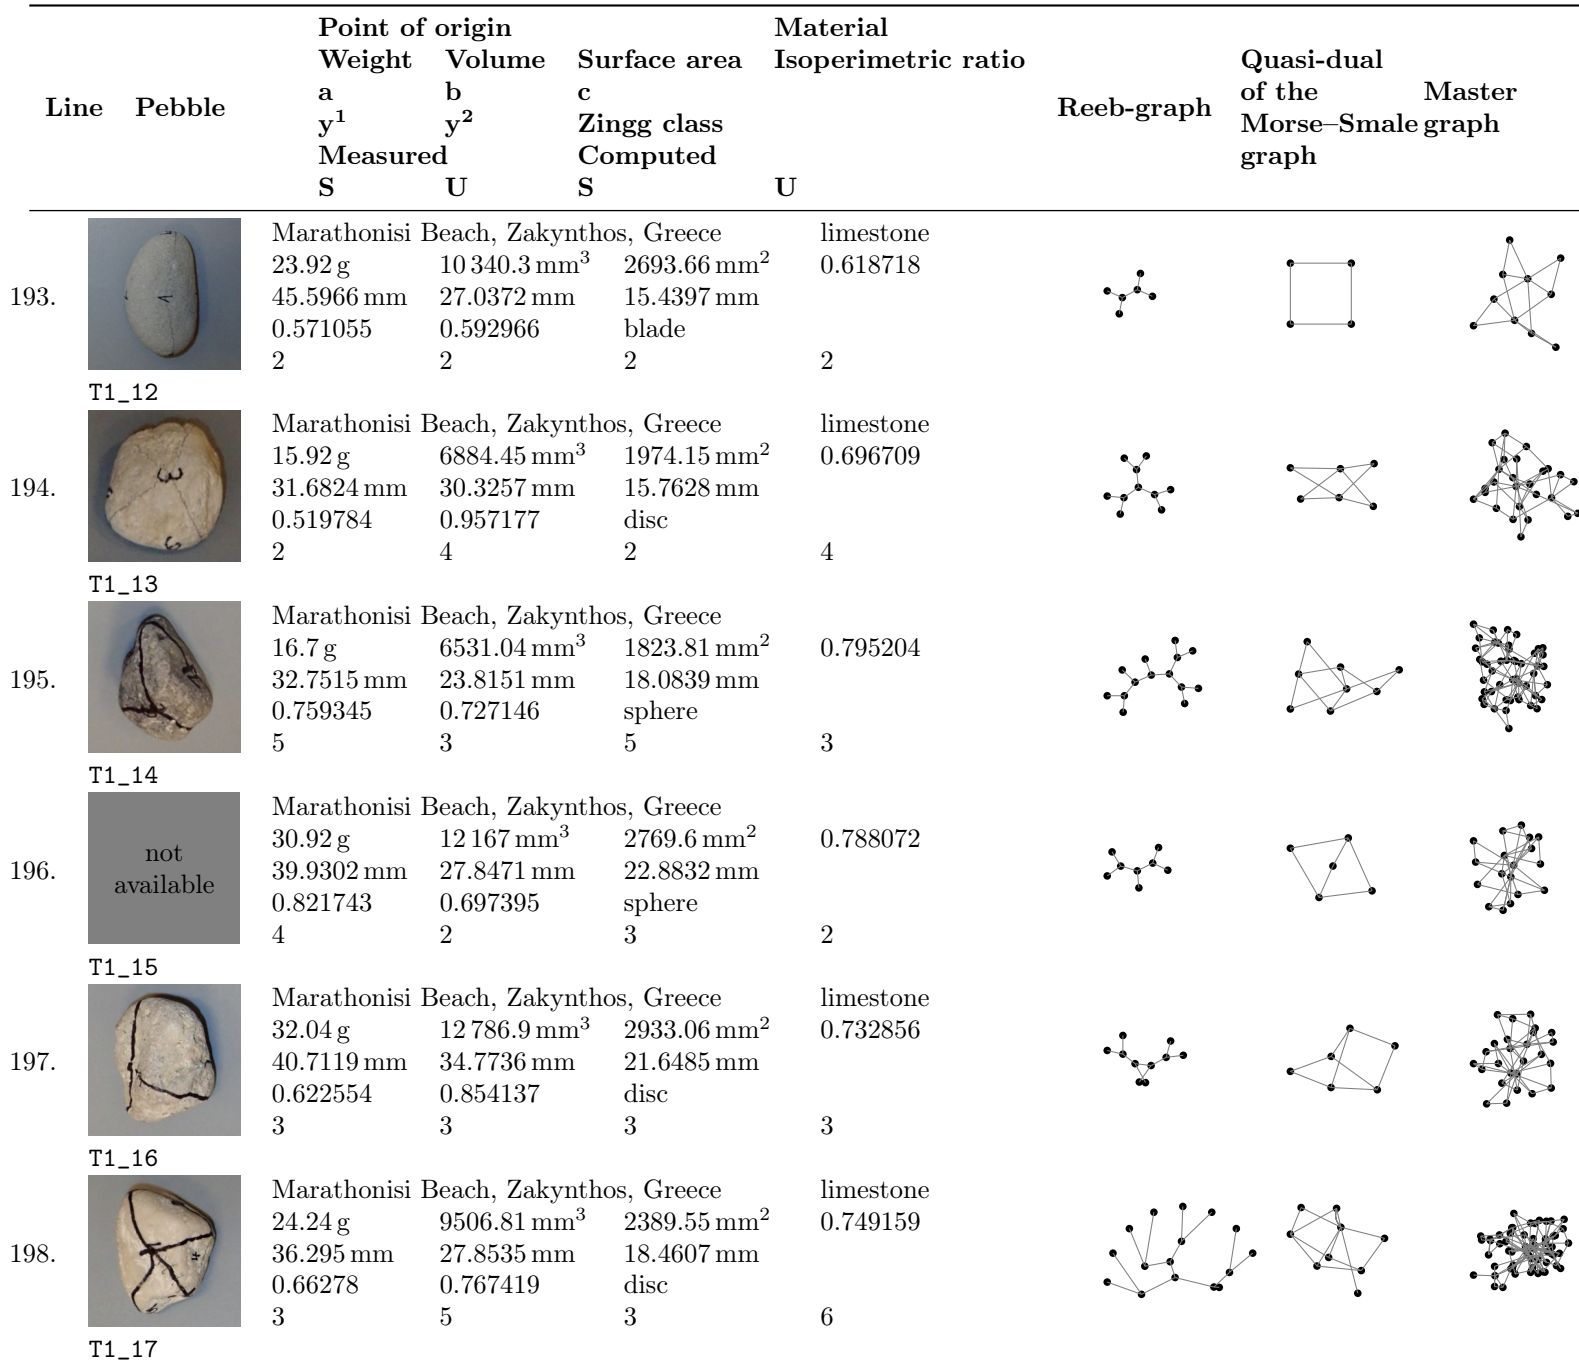   | Marathonisi Beach, Zakynthos, Greece<br>23.92 g<br>45.5966 mm<br>0.571055<br>2 | 23.92 g<br>10 340.3 mm <sup>3</sup><br>27.0372 mm<br>0.592966<br>2 | 2693.66 mm <sup>2</sup><br>15.4397 mm<br>blade<br>2  | limestone<br>0.618718<br><br>2 |                     | 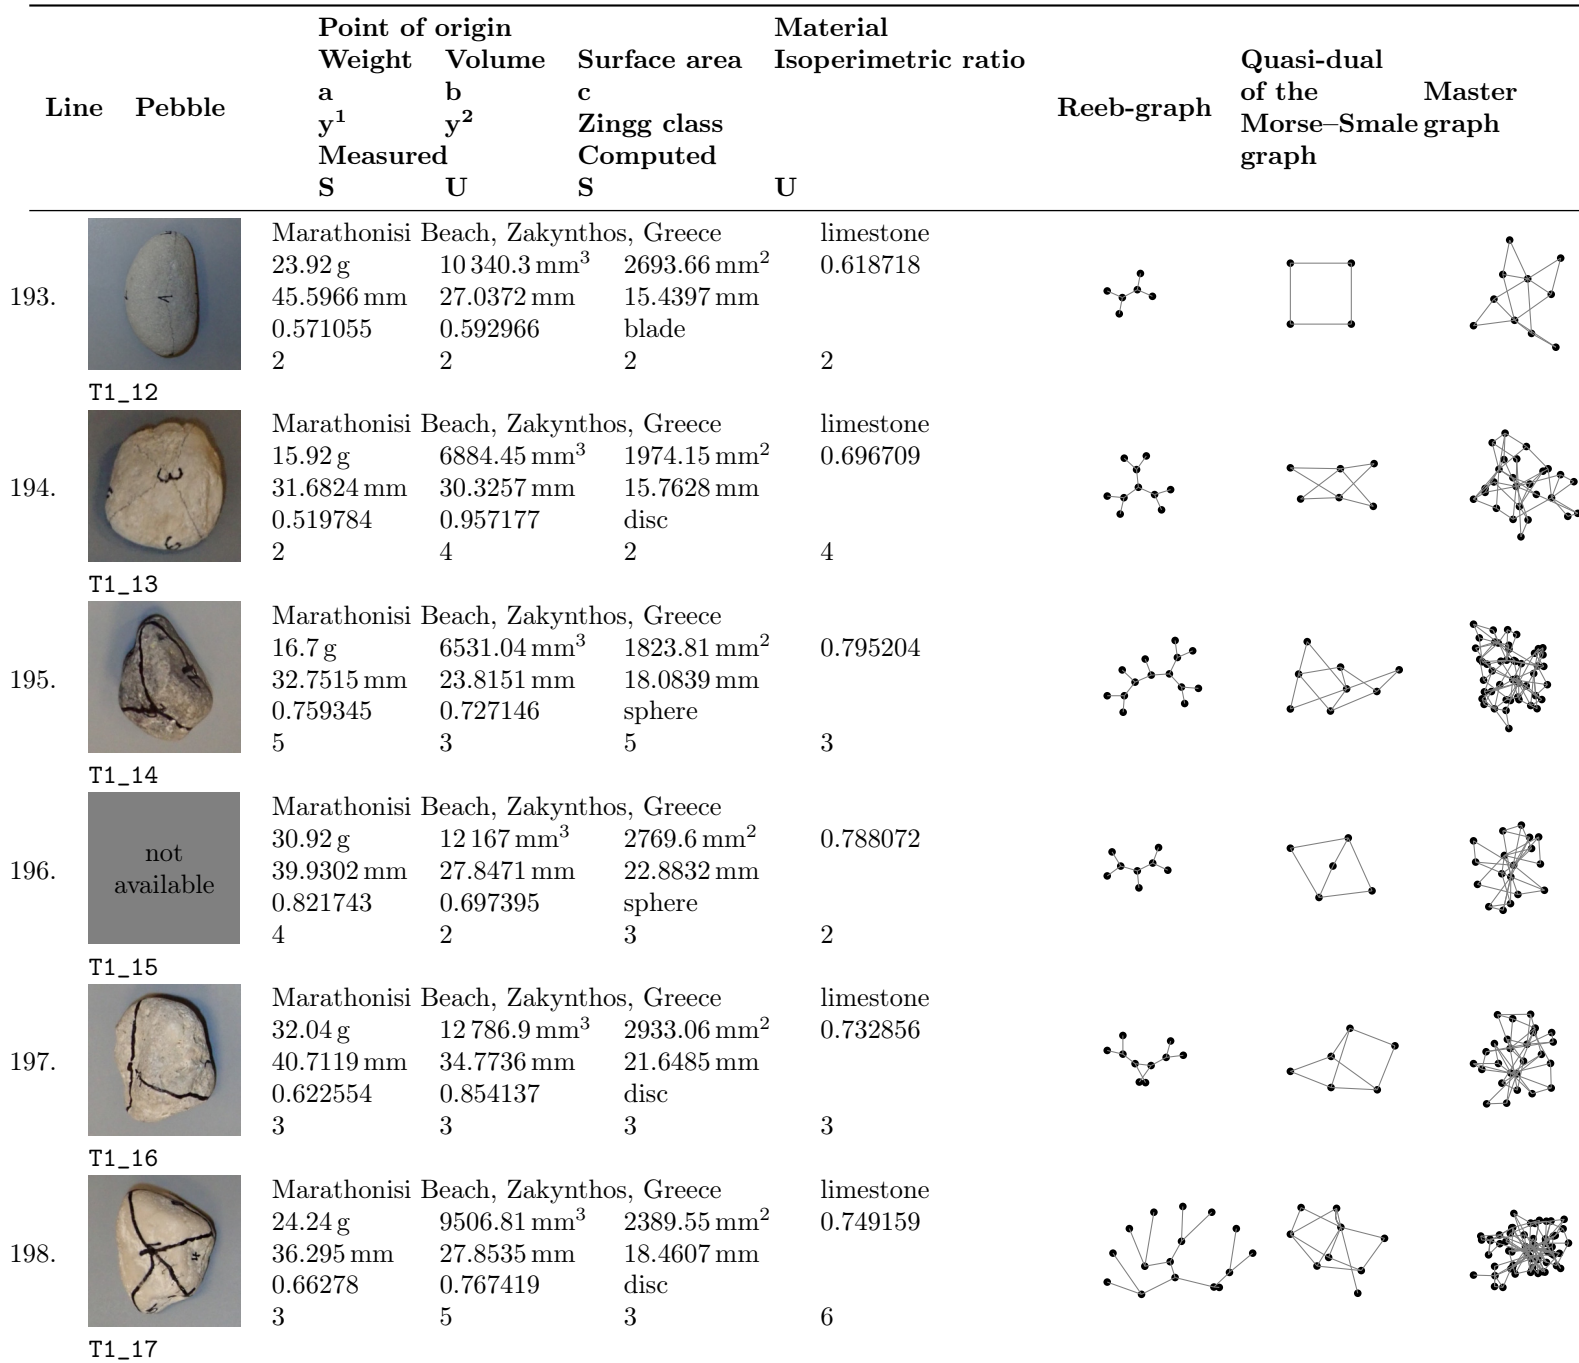   | 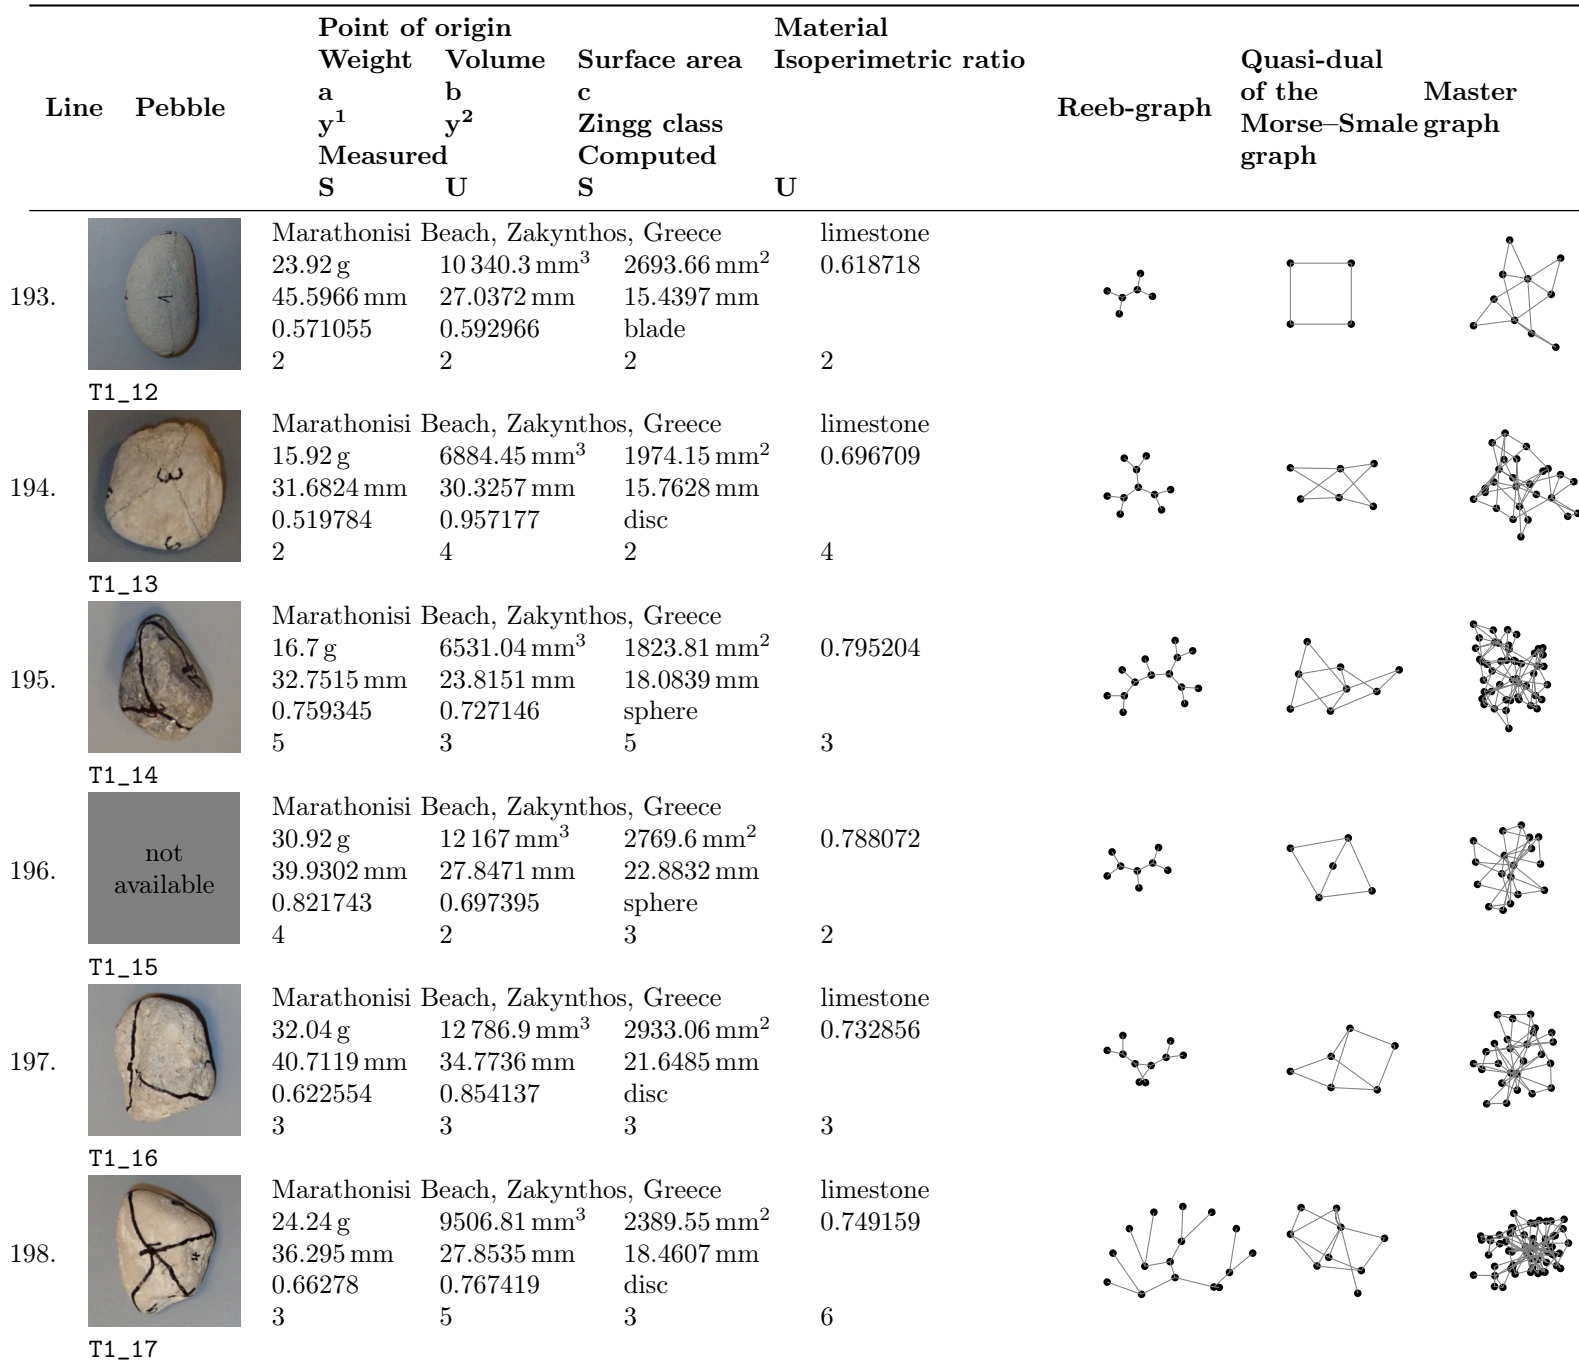   | 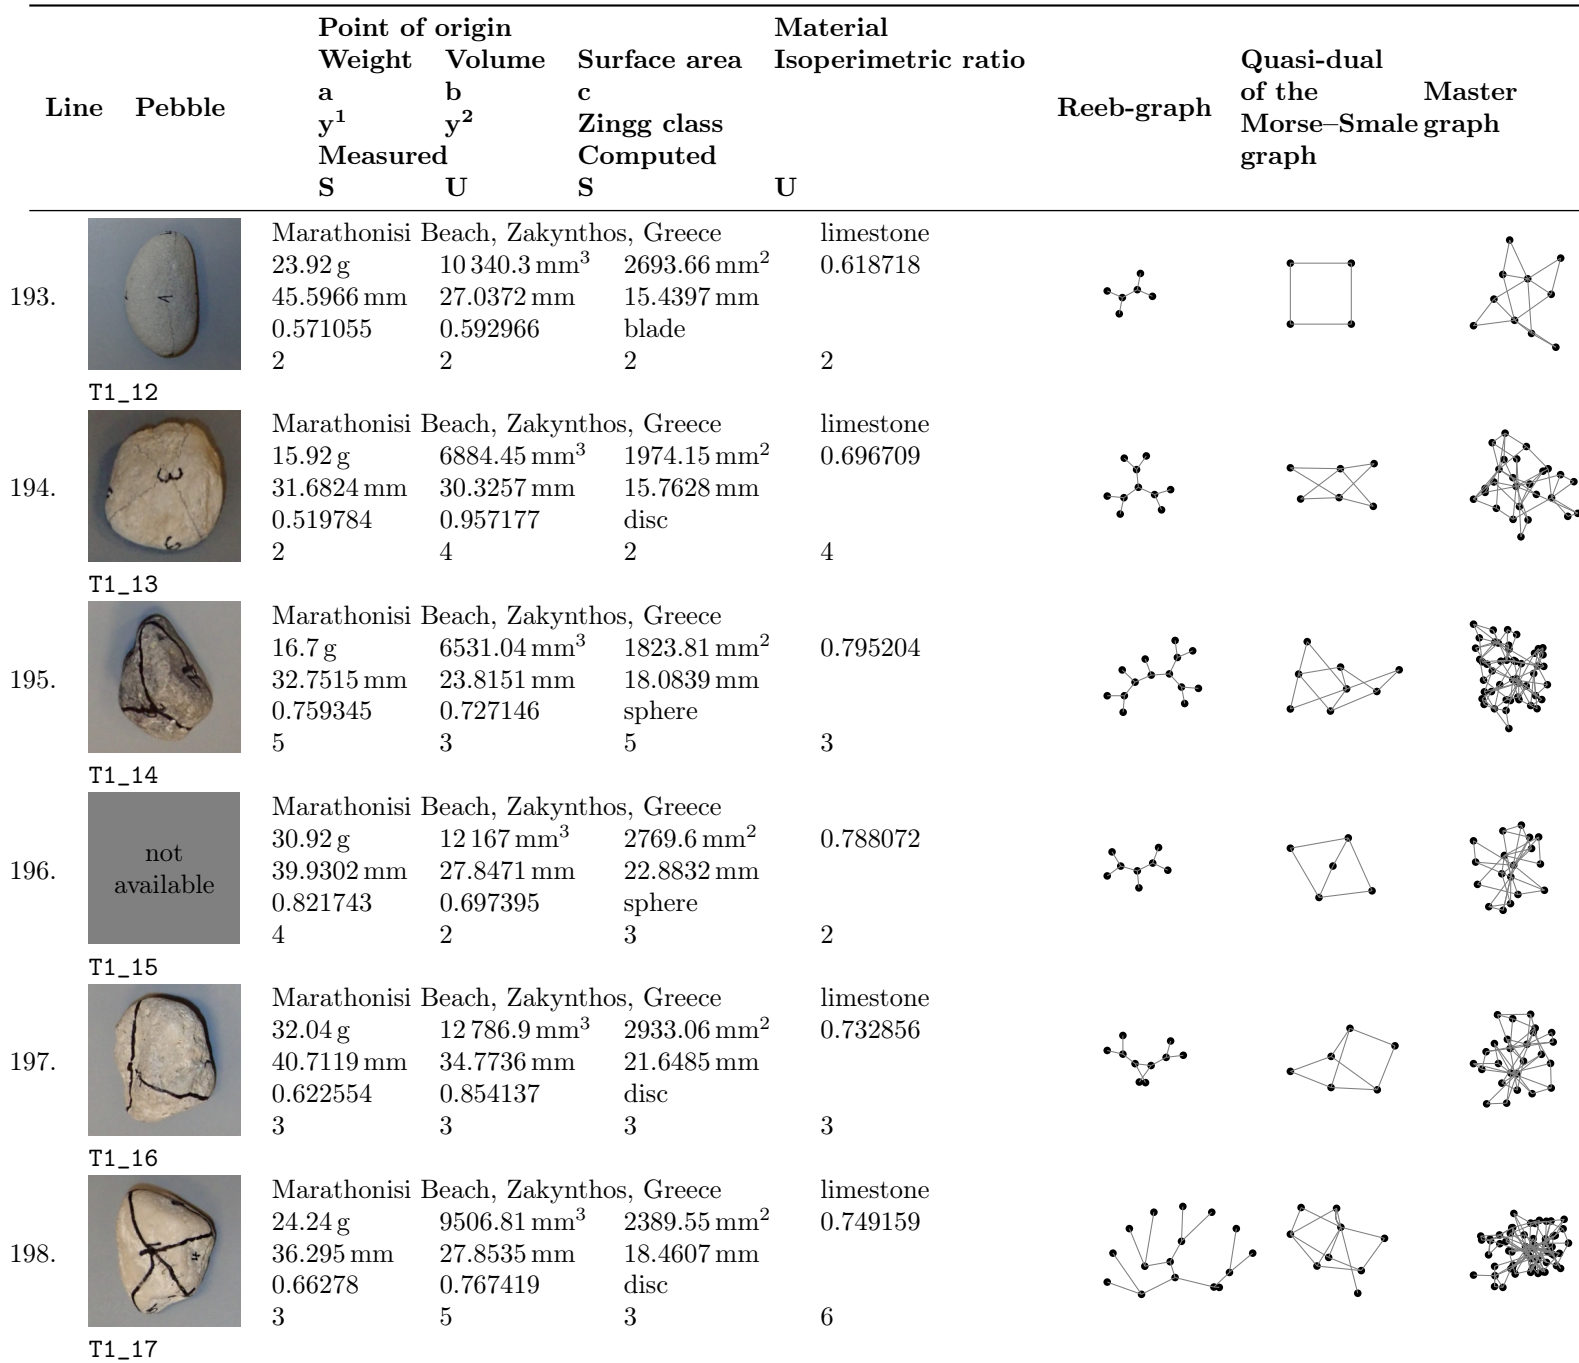   |
|      | T1_12                                                                               |                                                                                |                                                                    |                                                      |                                |                     |                                                                                       |                                                                                       |                                                                                       |
| 194. | 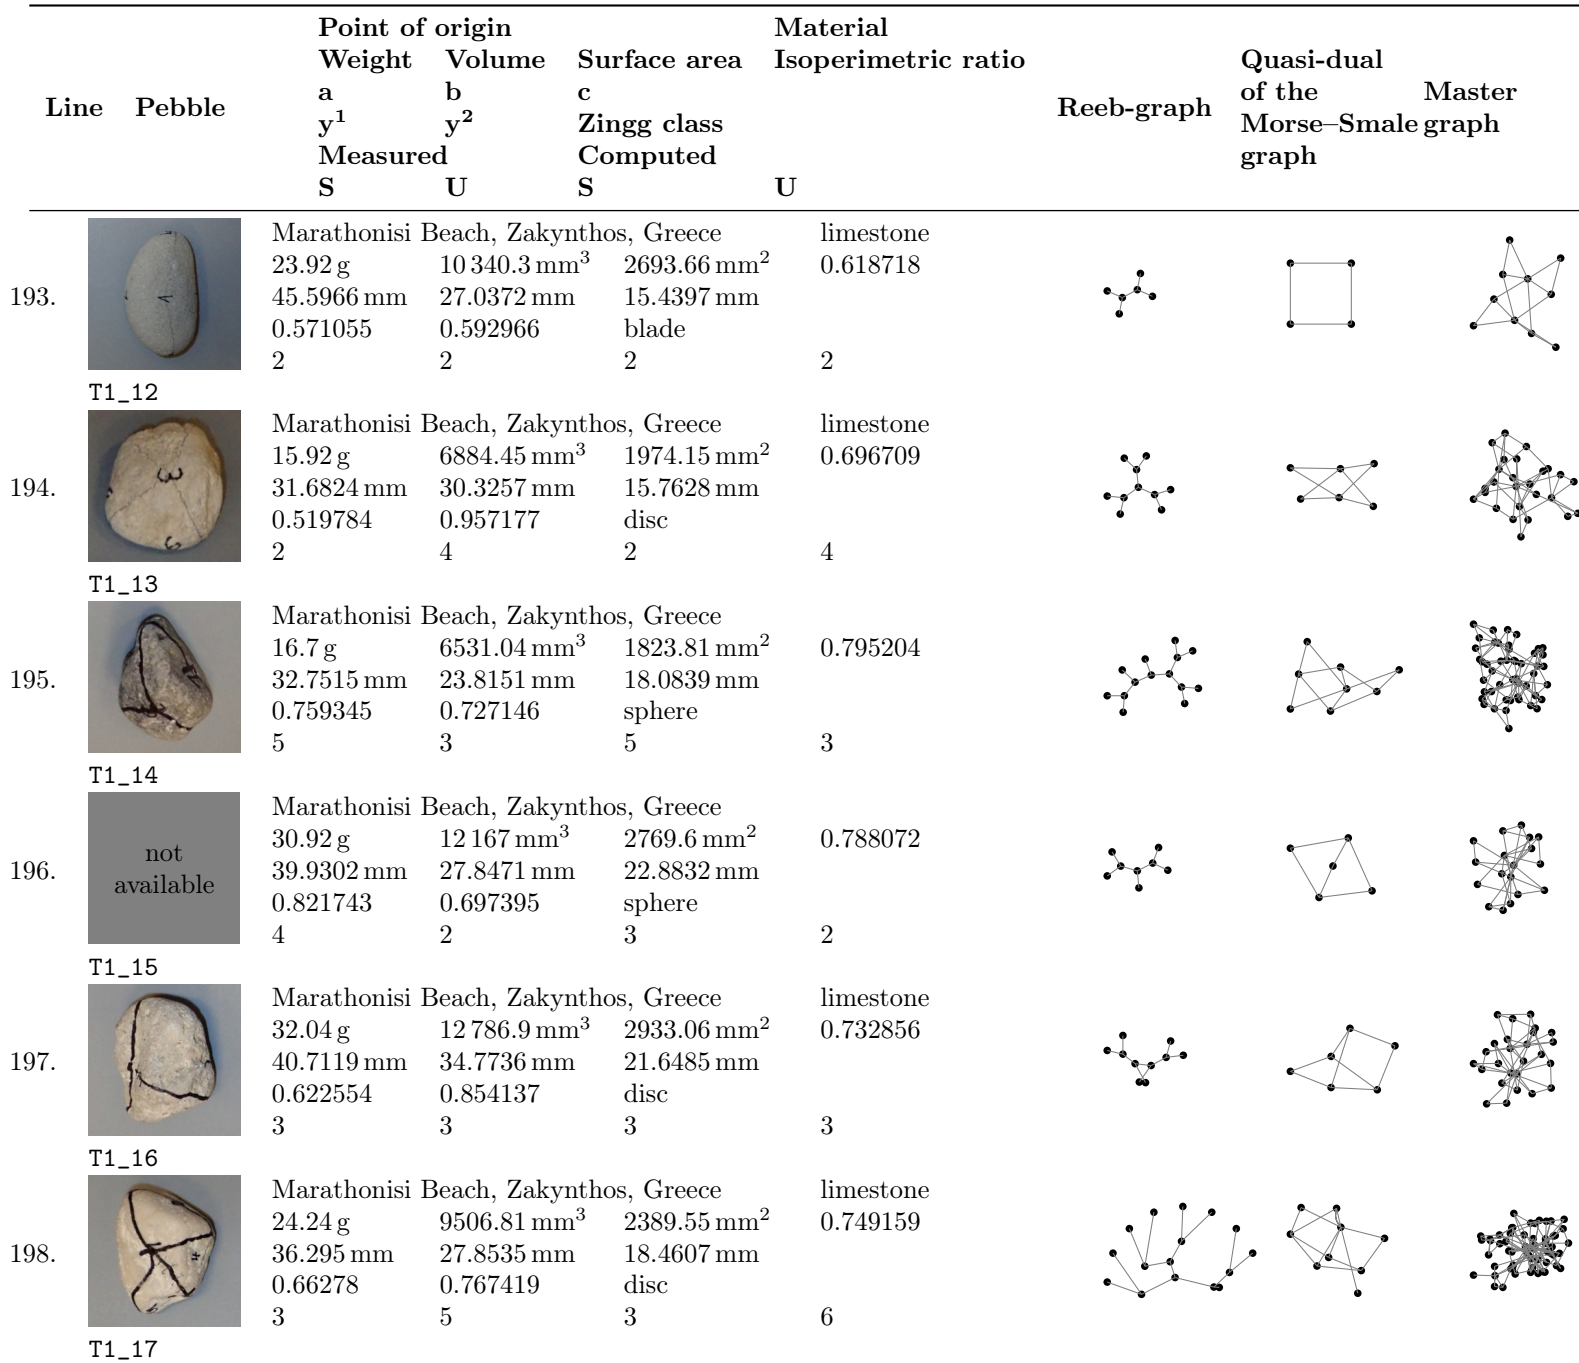   | Marathonisi Beach, Zakynthos, Greece<br>15.92 g<br>31.6824 mm<br>0.519784<br>2 | 15.92 g<br>6884.45 mm <sup>3</sup><br>30.3257 mm<br>0.957177<br>4  | 1974.15 mm <sup>2</sup><br>15.7628 mm<br>disc<br>2   | limestone<br>0.696709<br><br>4 |                     | 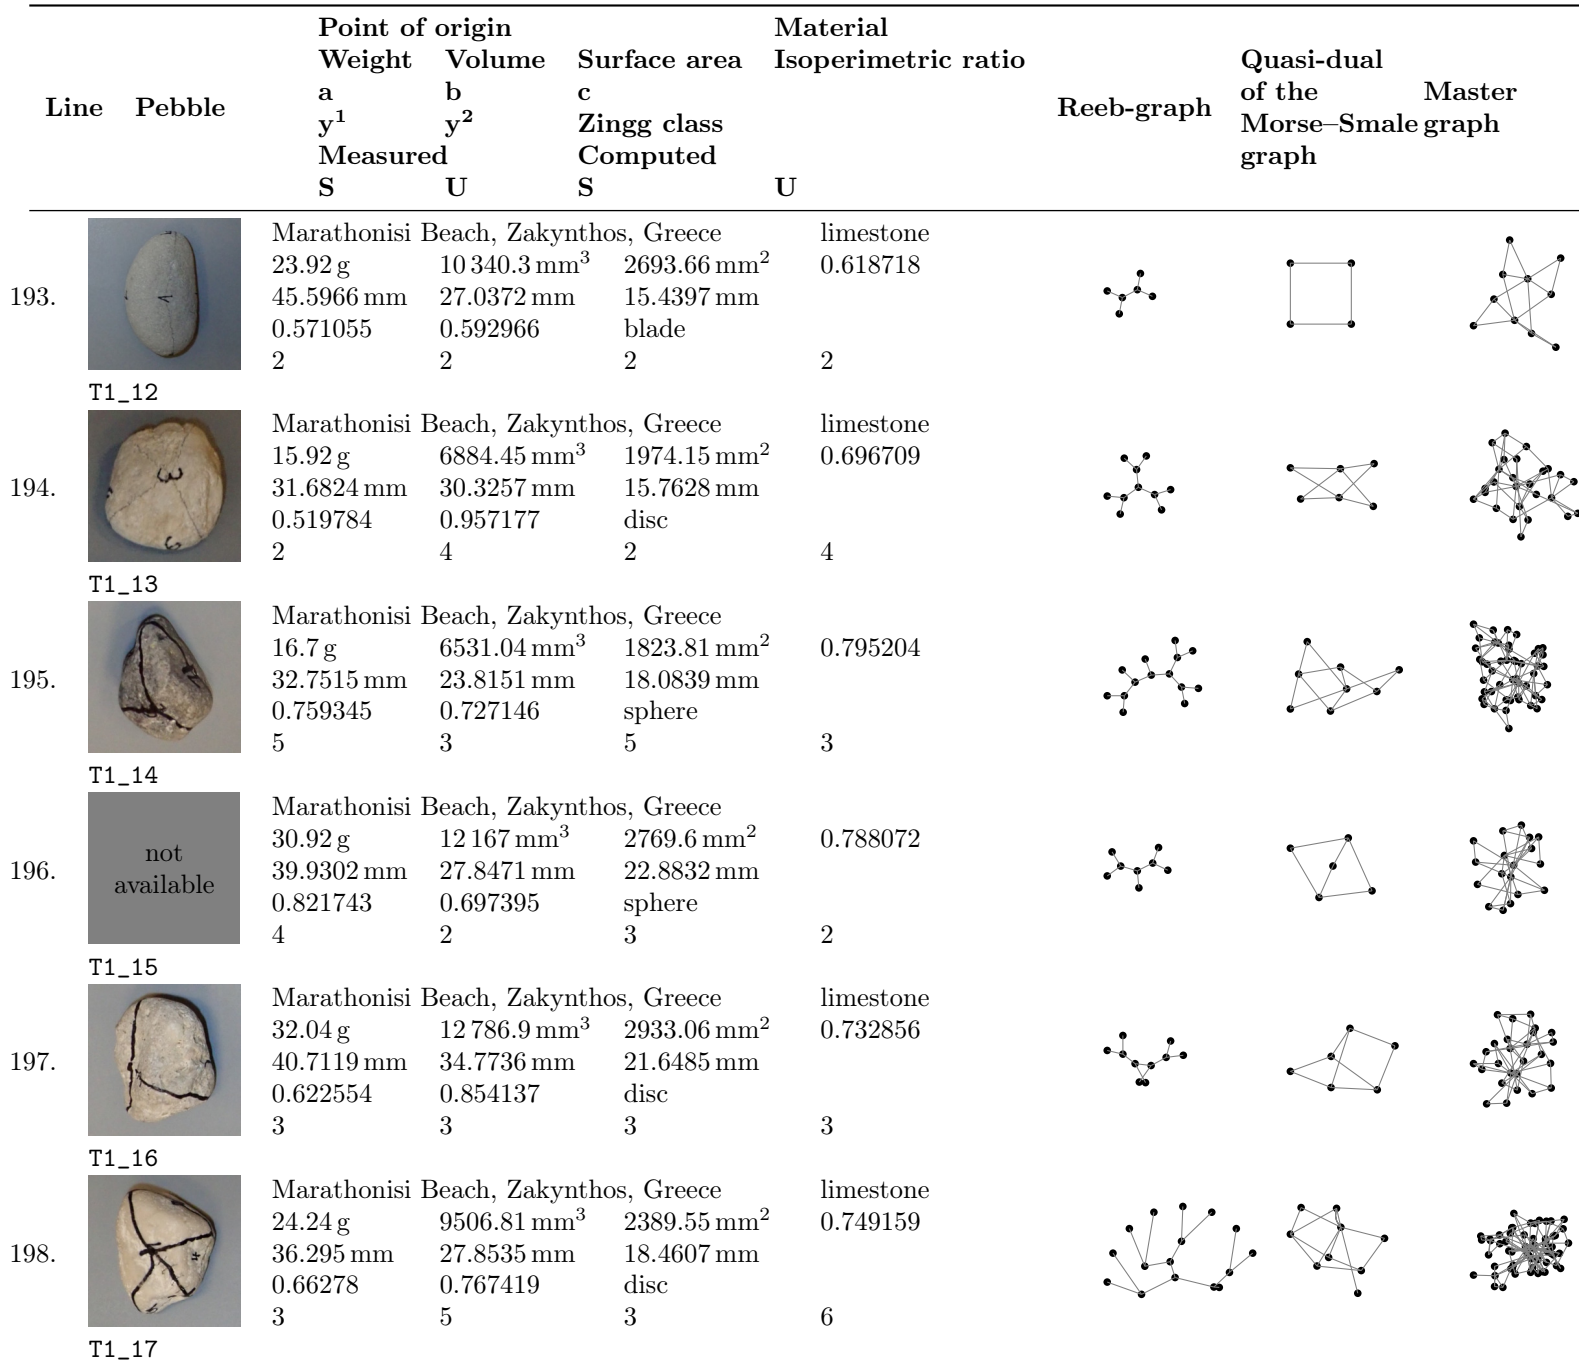   | 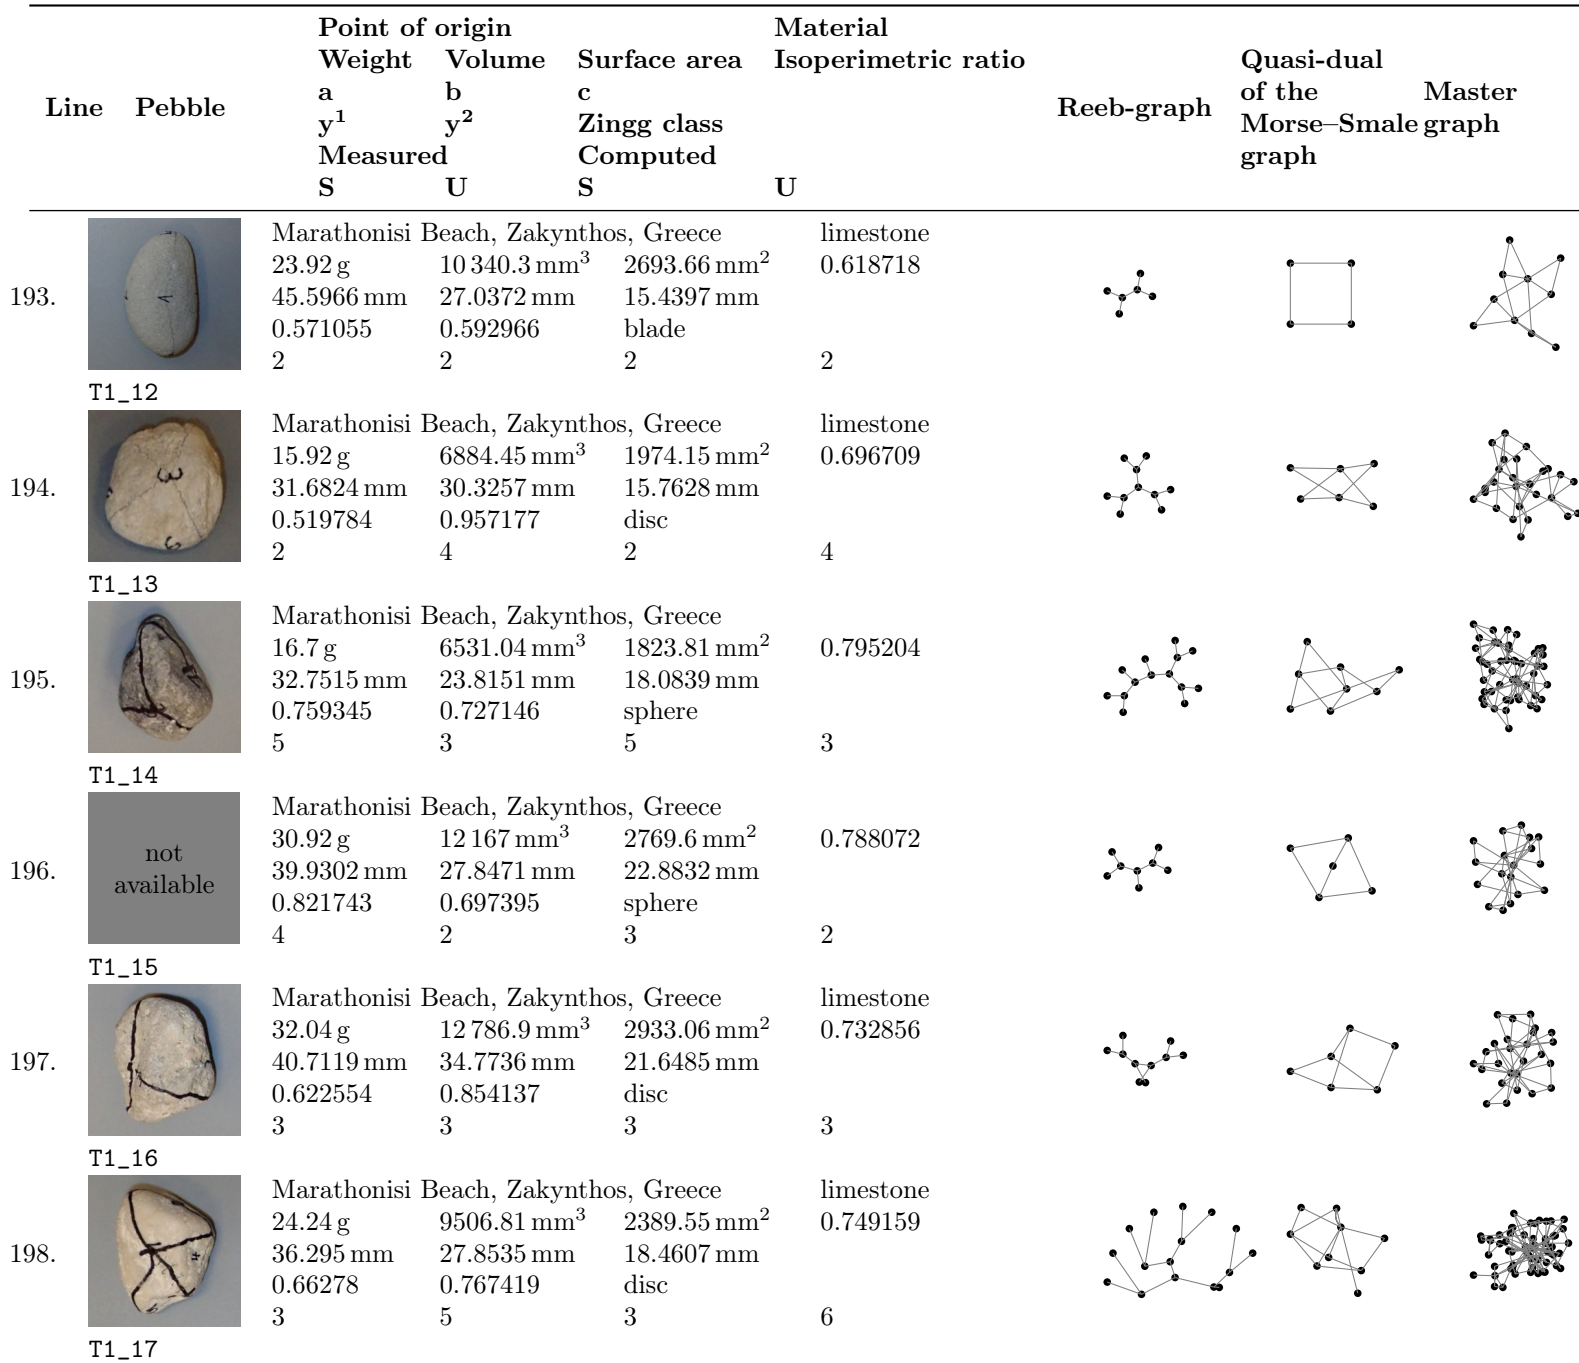   | 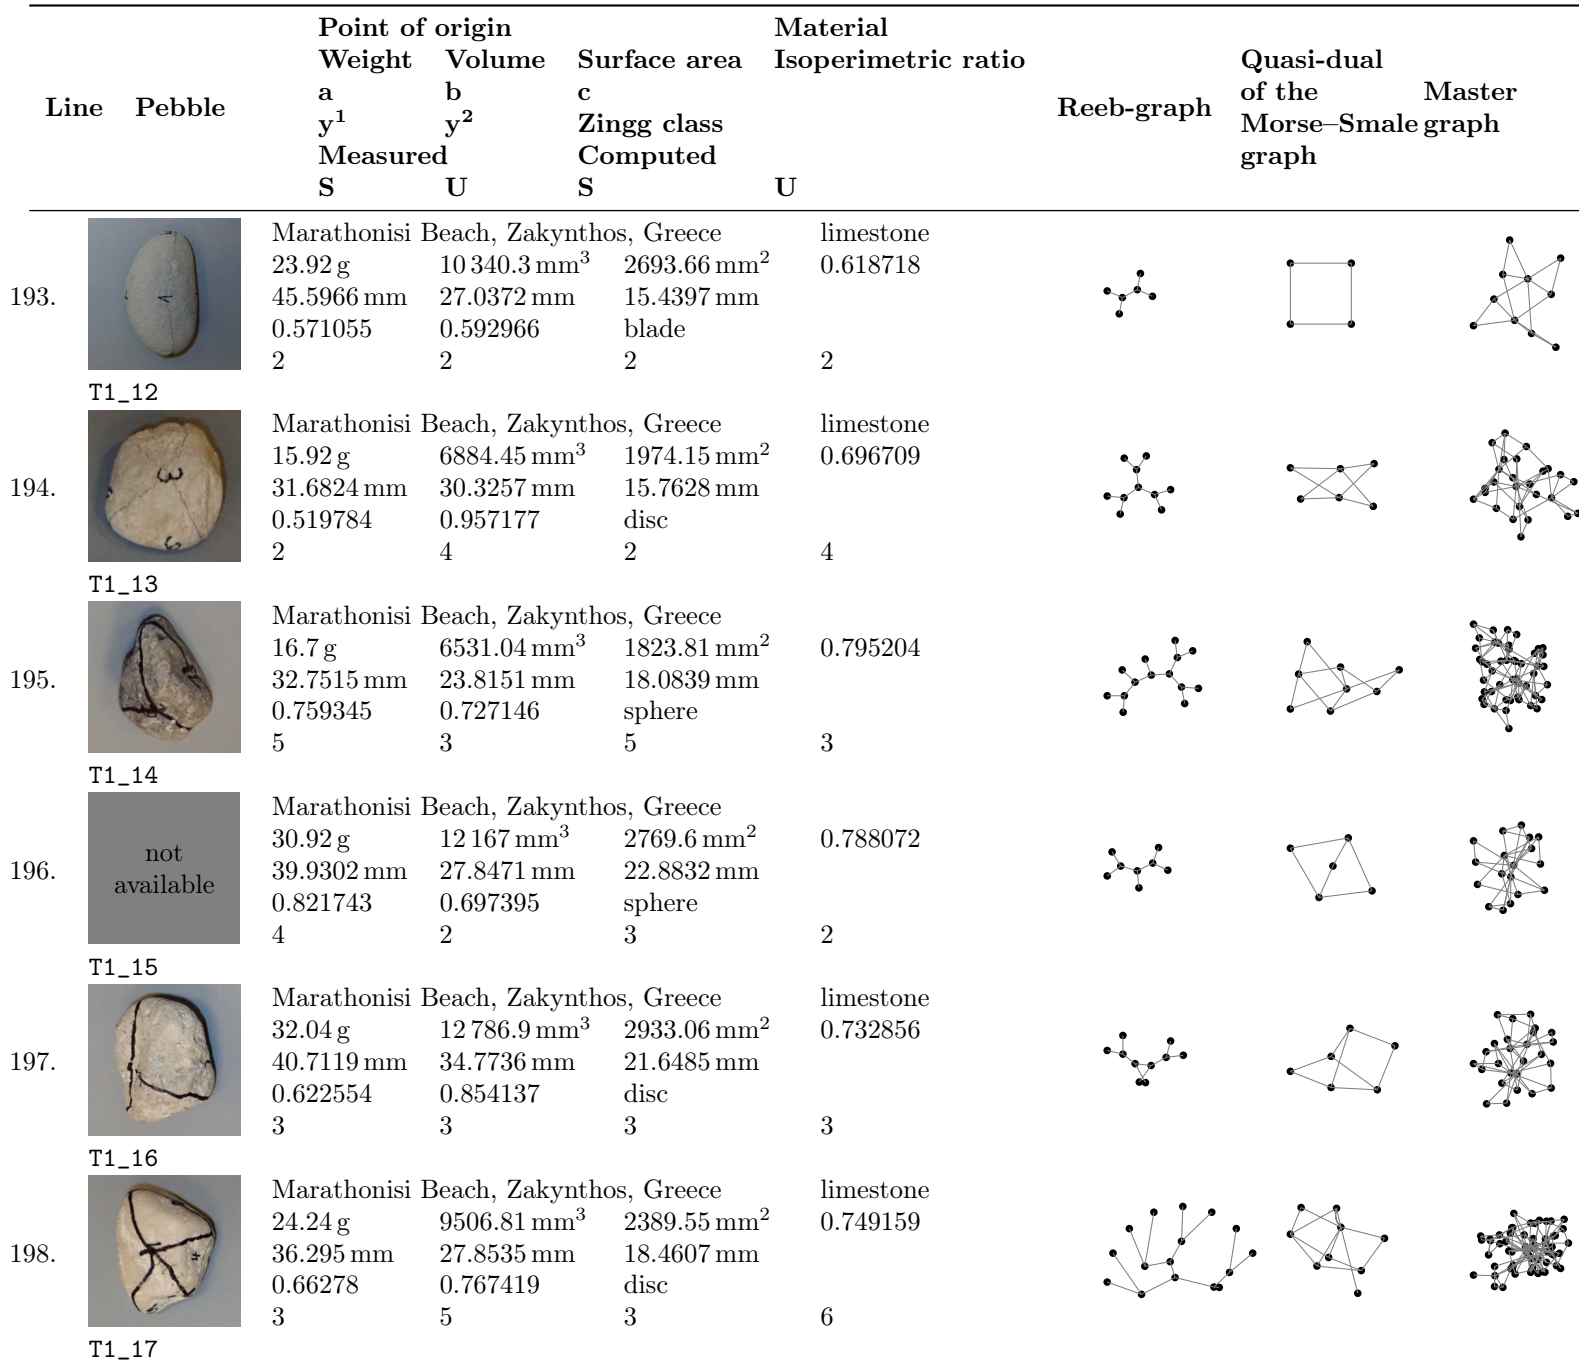   |
|      | T1_13                                                                               |                                                                                |                                                                    |                                                      |                                |                     |                                                                                       |                                                                                       |                                                                                       |
| 195. | 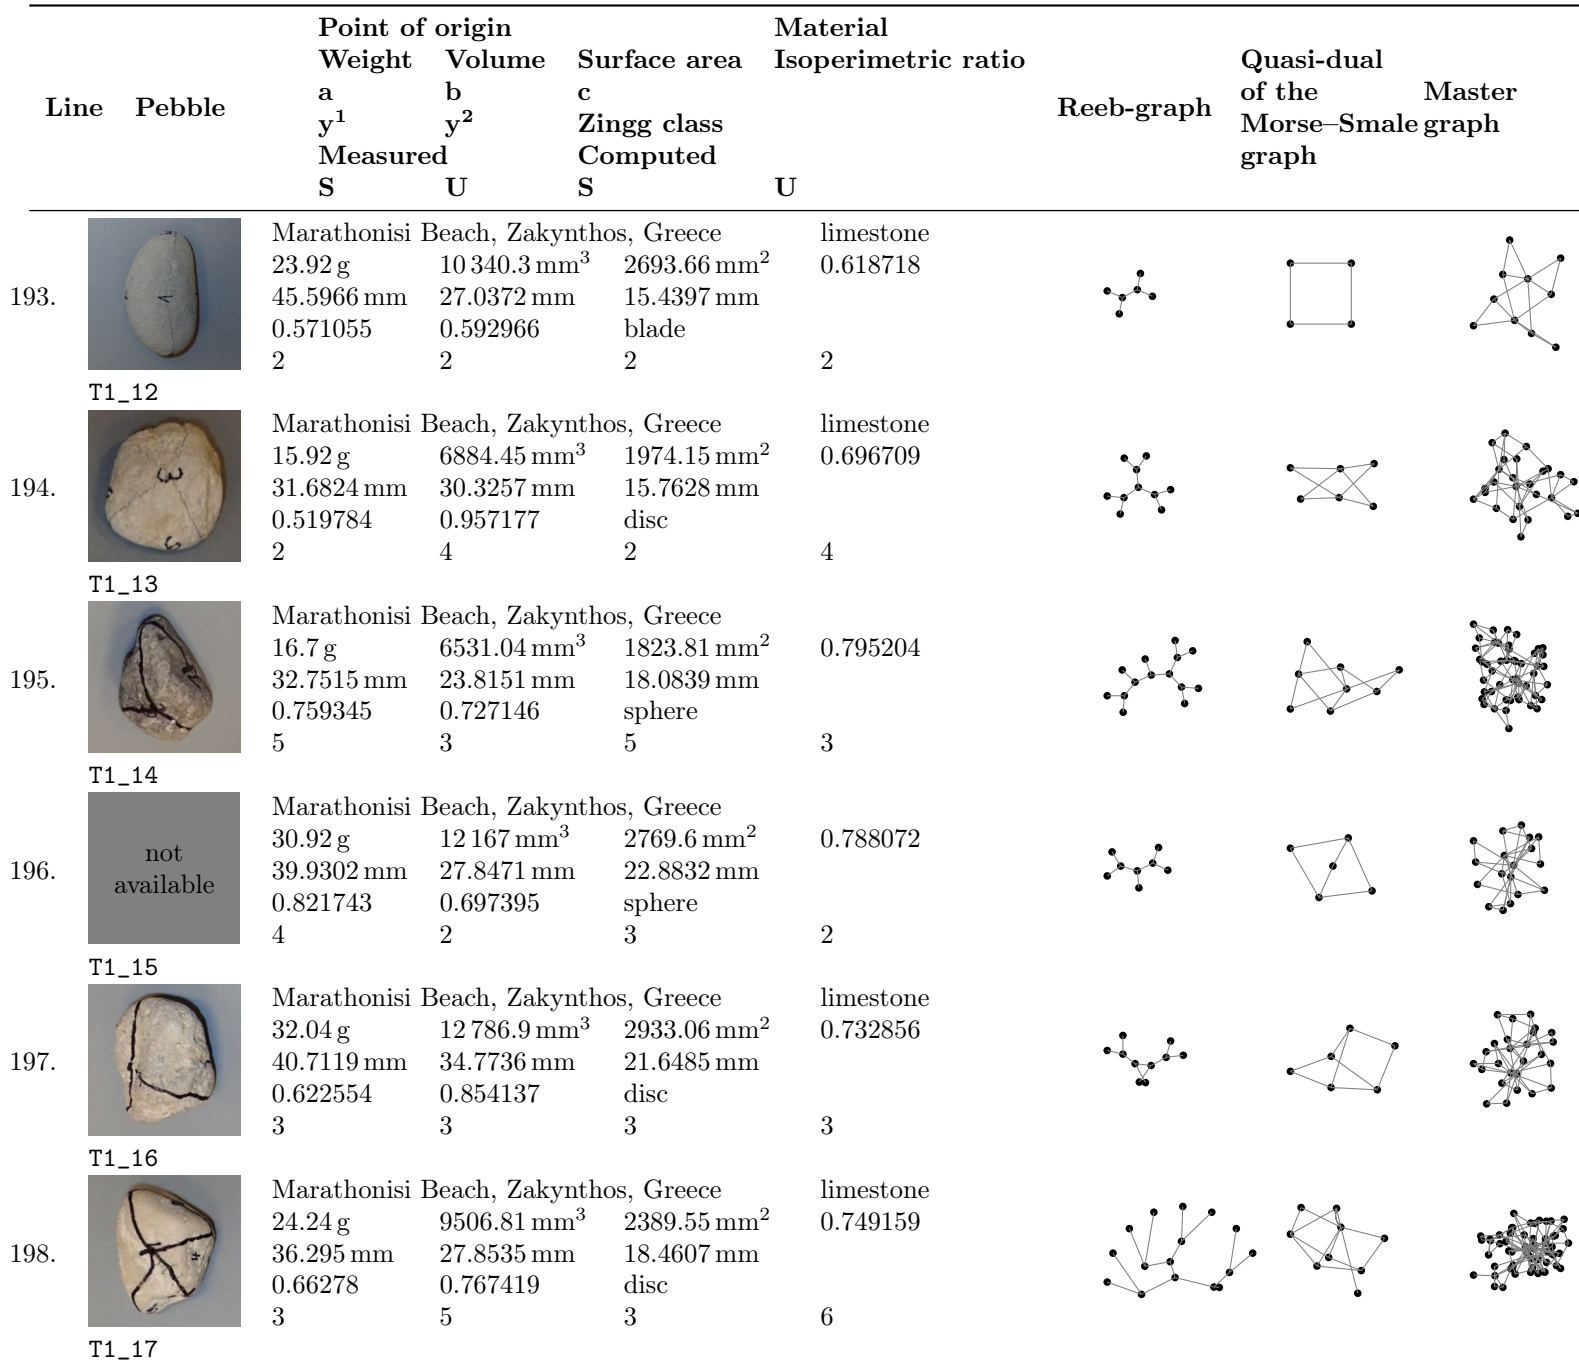   | Marathonisi Beach, Zakynthos, Greece<br>16.7 g<br>32.7515 mm<br>0.759345<br>5  | 16.7 g<br>6531.04 mm <sup>3</sup><br>23.8151 mm<br>0.727146<br>3   | 1823.81 mm <sup>2</sup><br>18.0839 mm<br>sphere<br>5 | 0.795204<br><br>3              |                     | 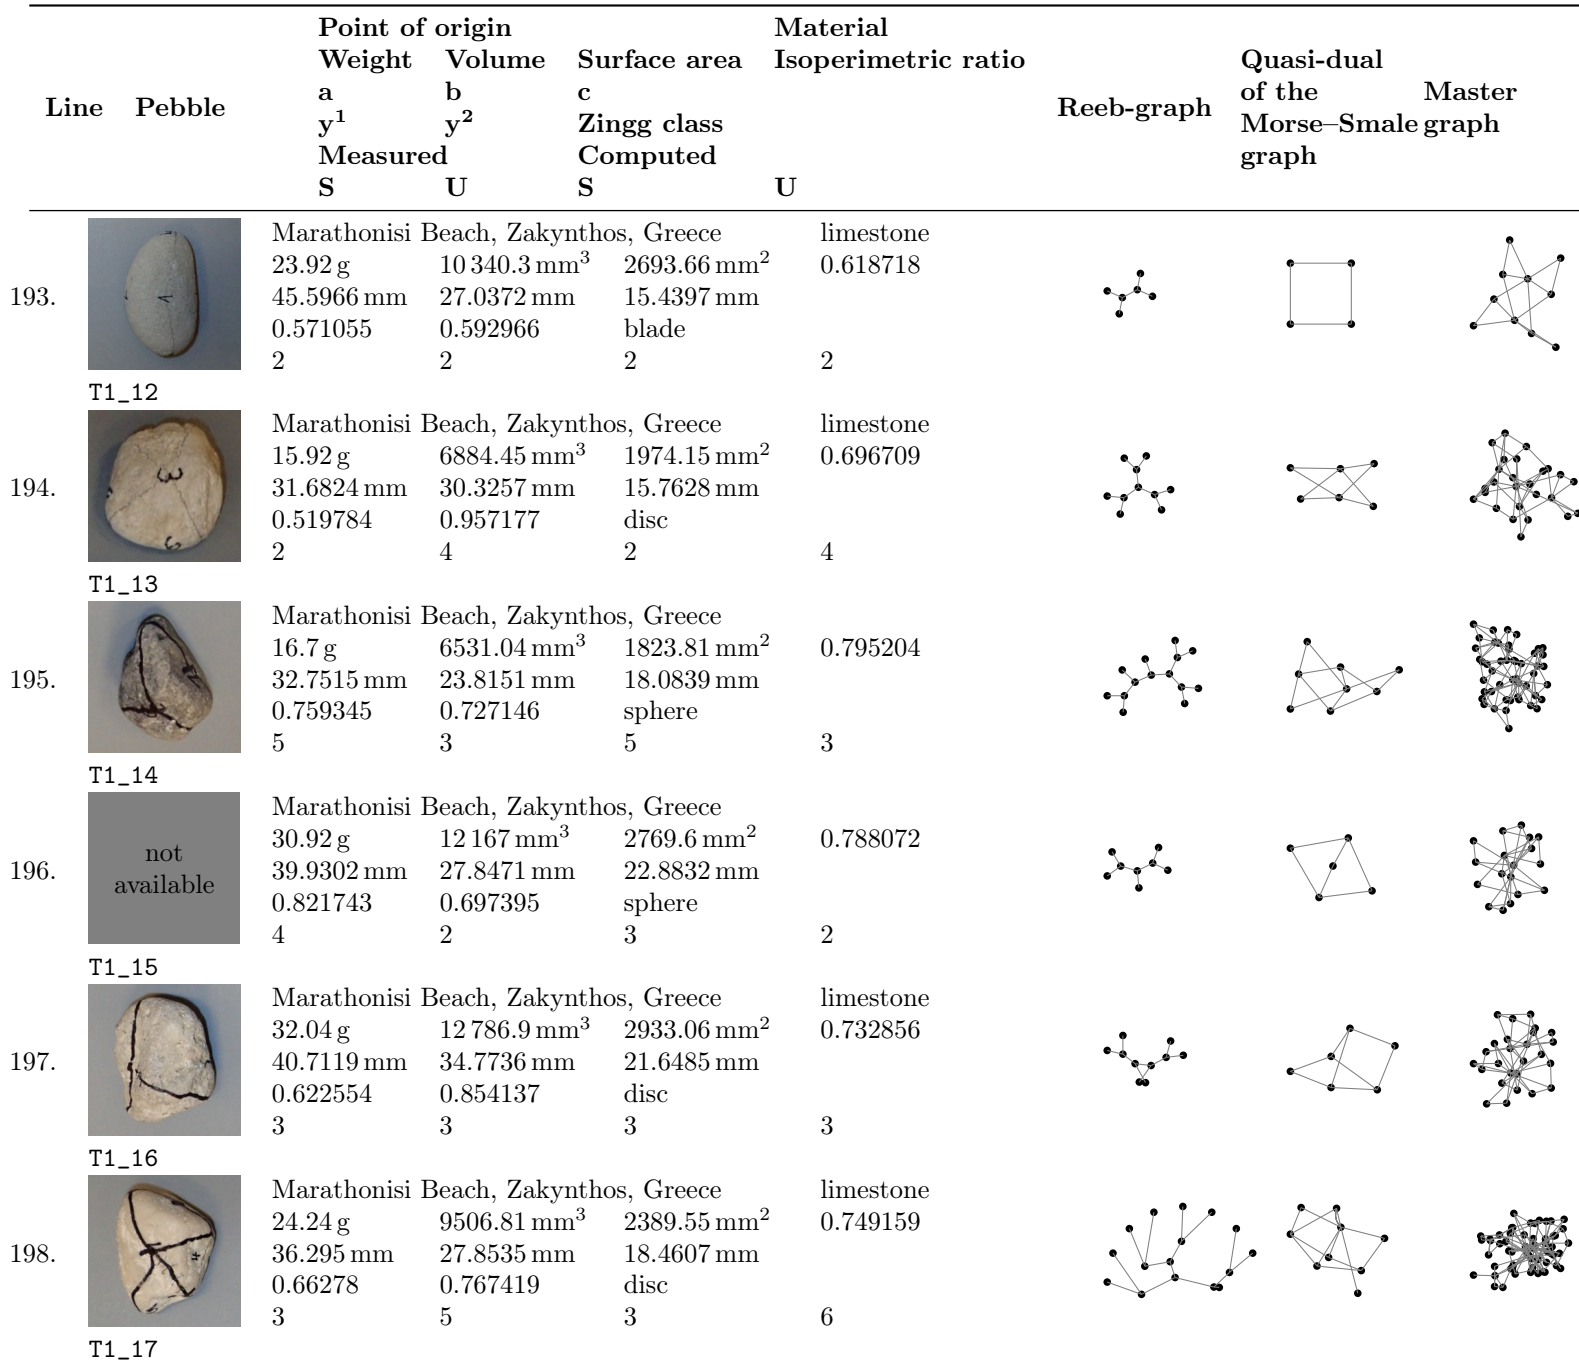   | 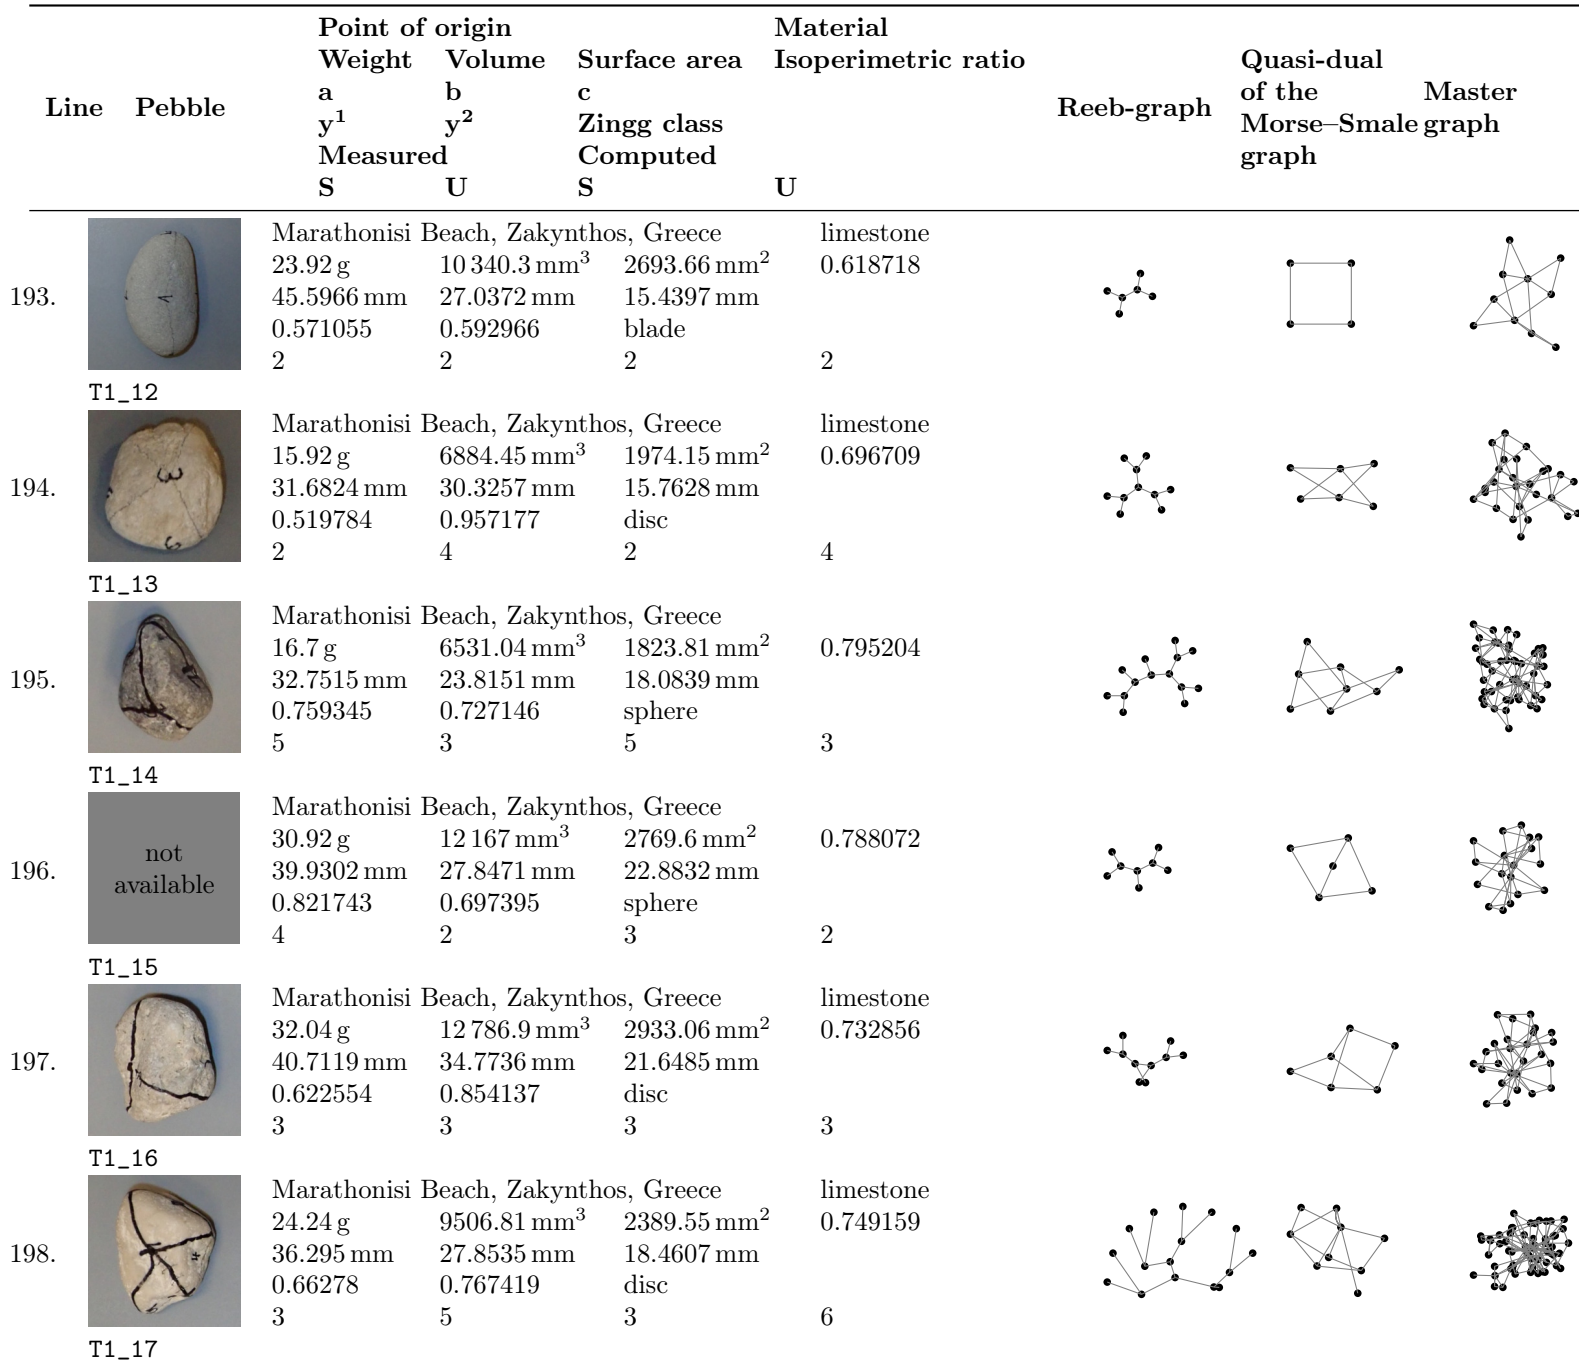   | 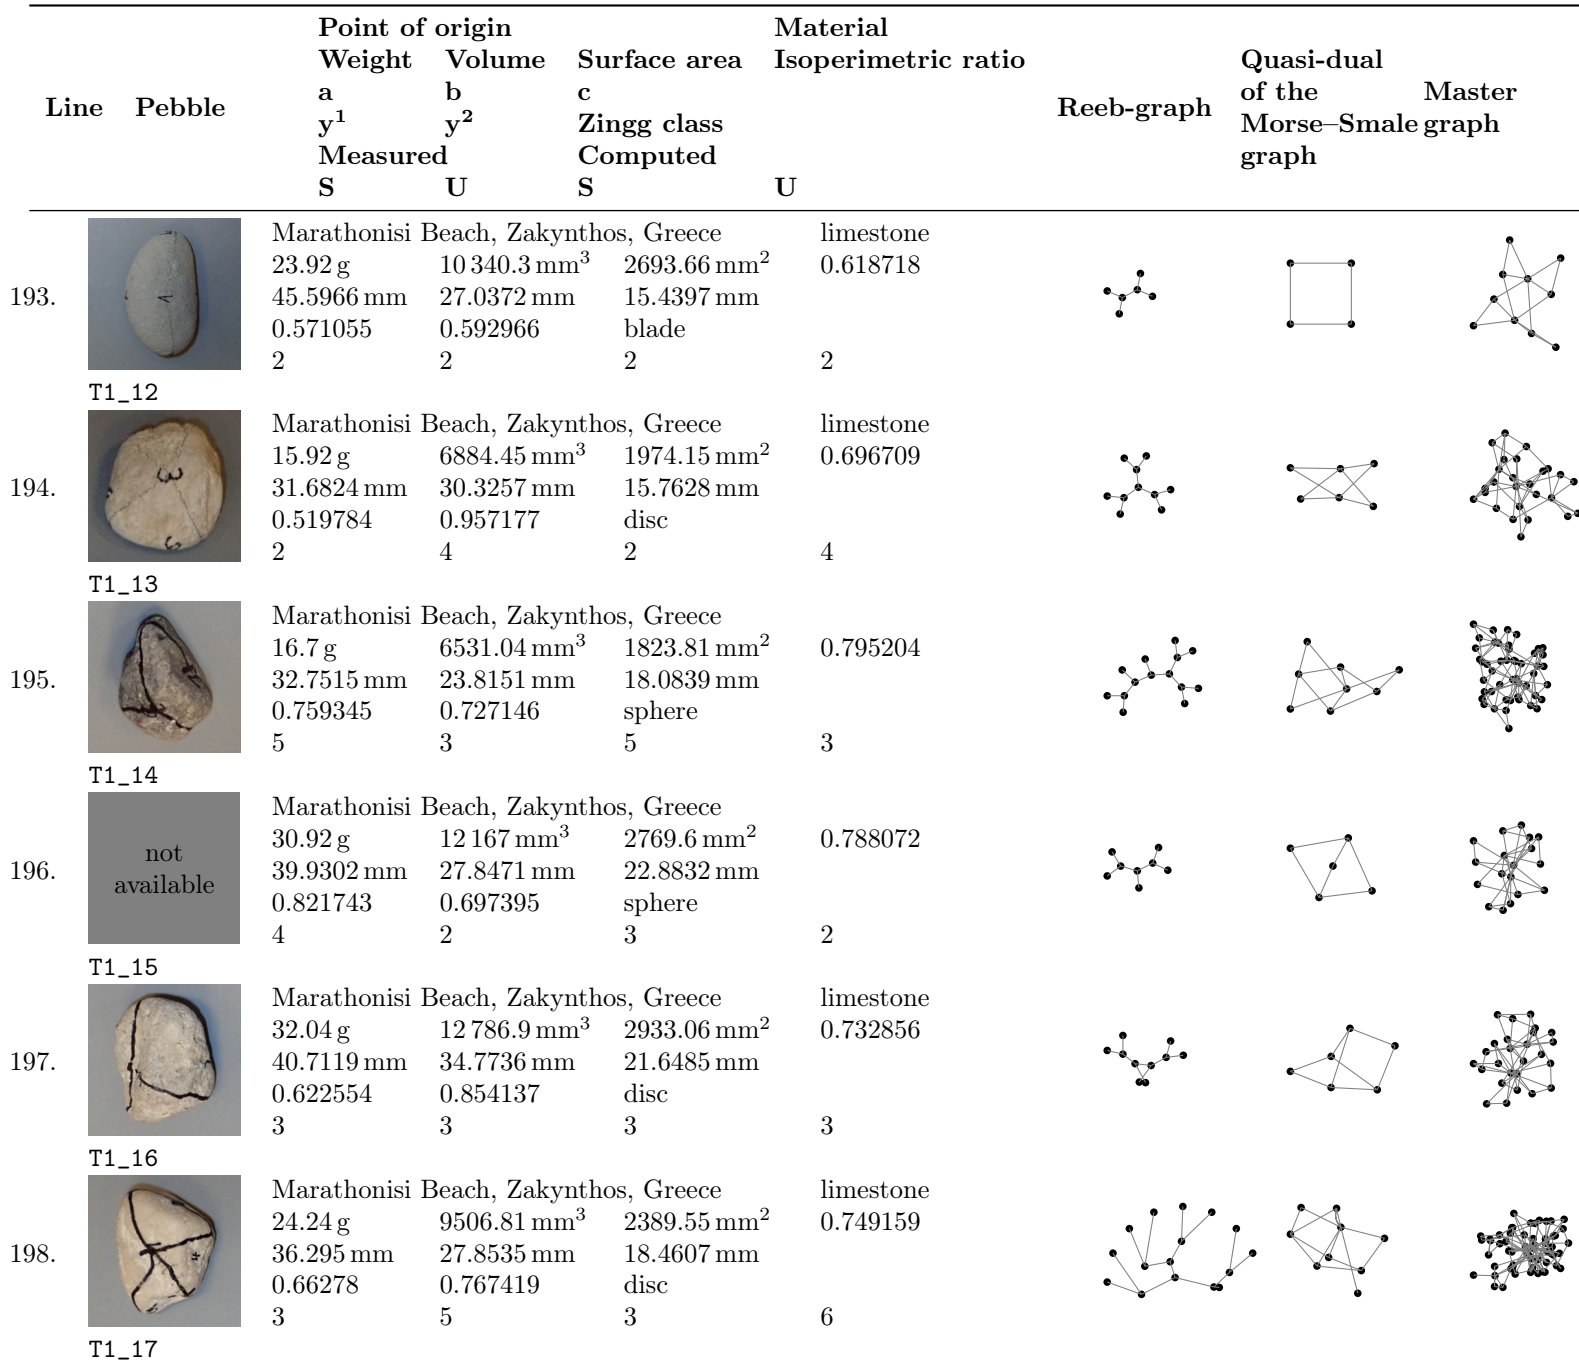   |
|      | T1_14                                                                               |                                                                                |                                                                    |                                                      |                                |                     |                                                                                       |                                                                                       |                                                                                       |
| 196. | 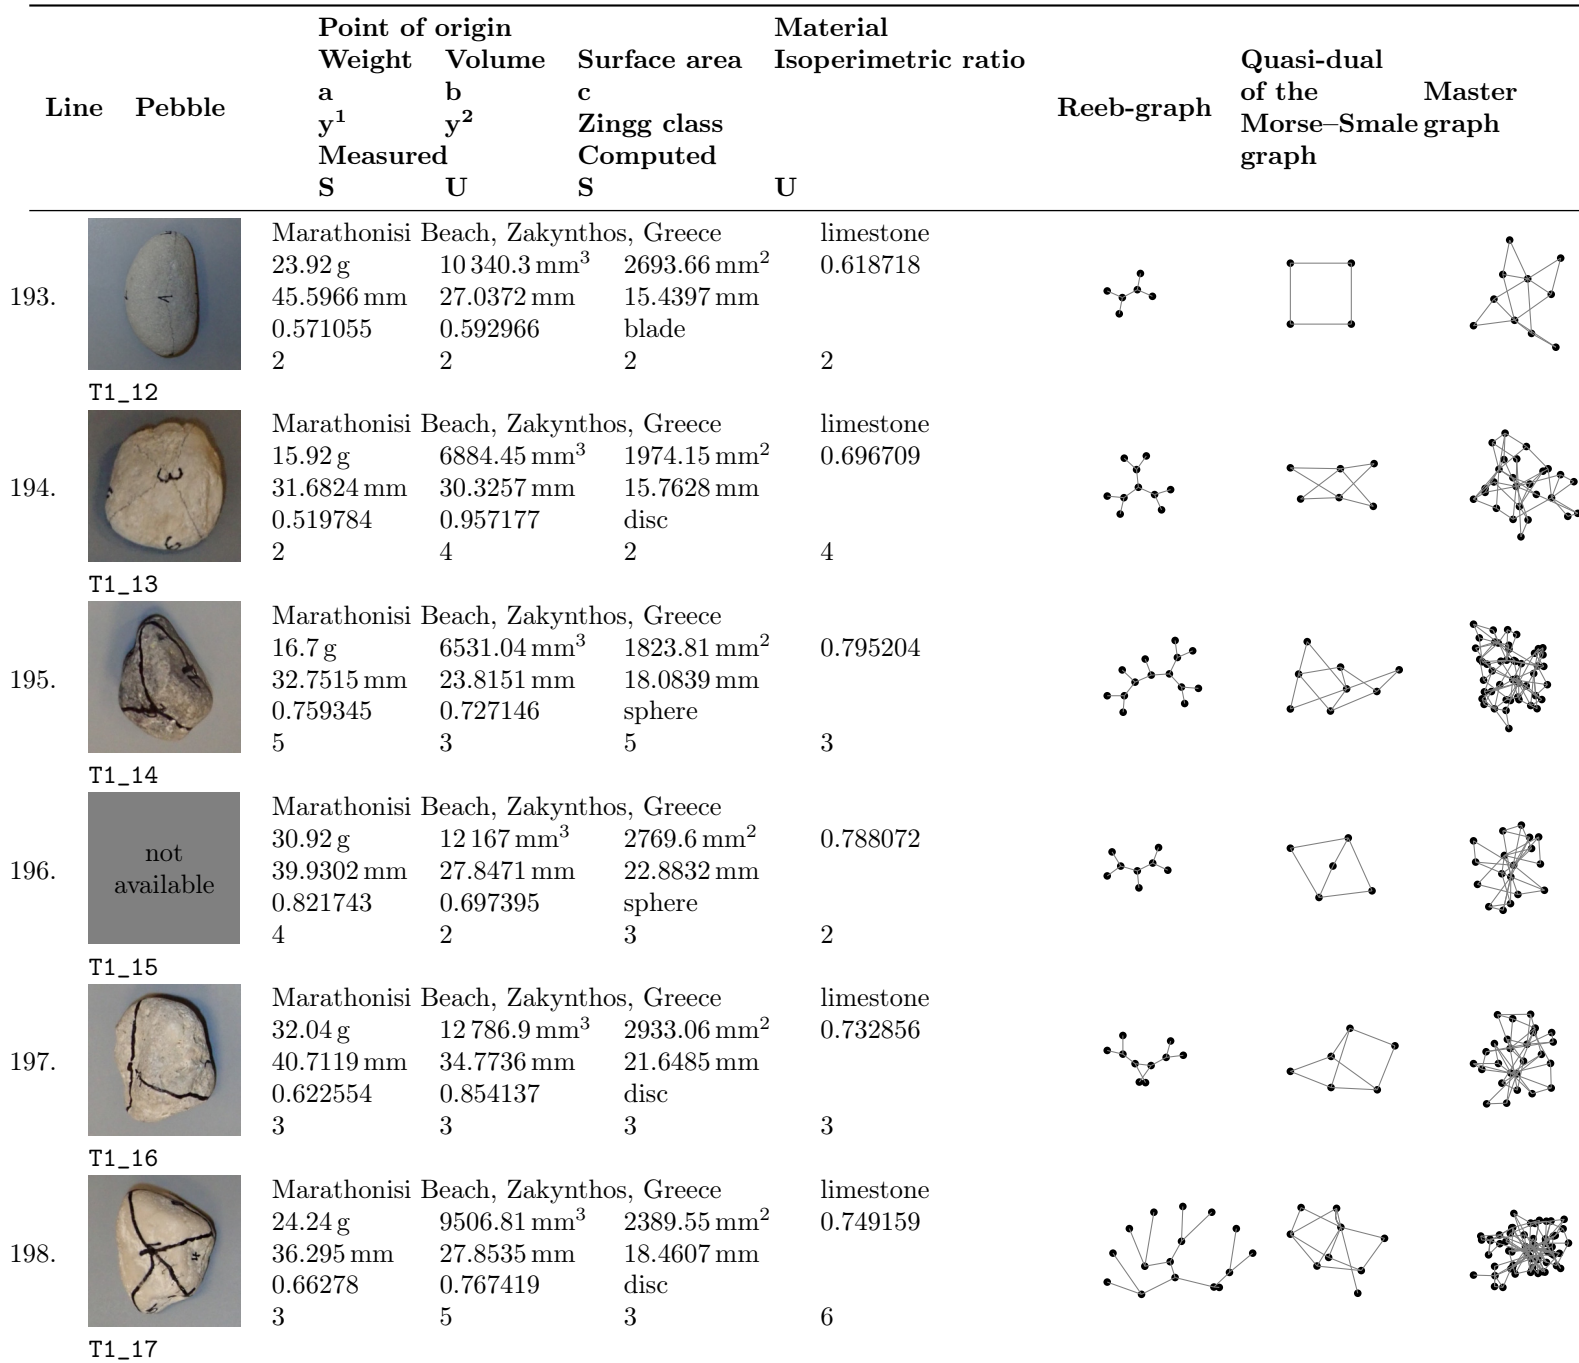  | Marathonisi Beach, Zakynthos, Greece<br>30.92 g<br>39.9302 mm<br>0.821743<br>4 | 30.92 g<br>12 167 mm <sup>3</sup><br>27.8471 mm<br>0.697395<br>2   | 2769.6 mm <sup>2</sup><br>22.8832 mm<br>sphere<br>3  | 0.788072<br><br>2              |                     | 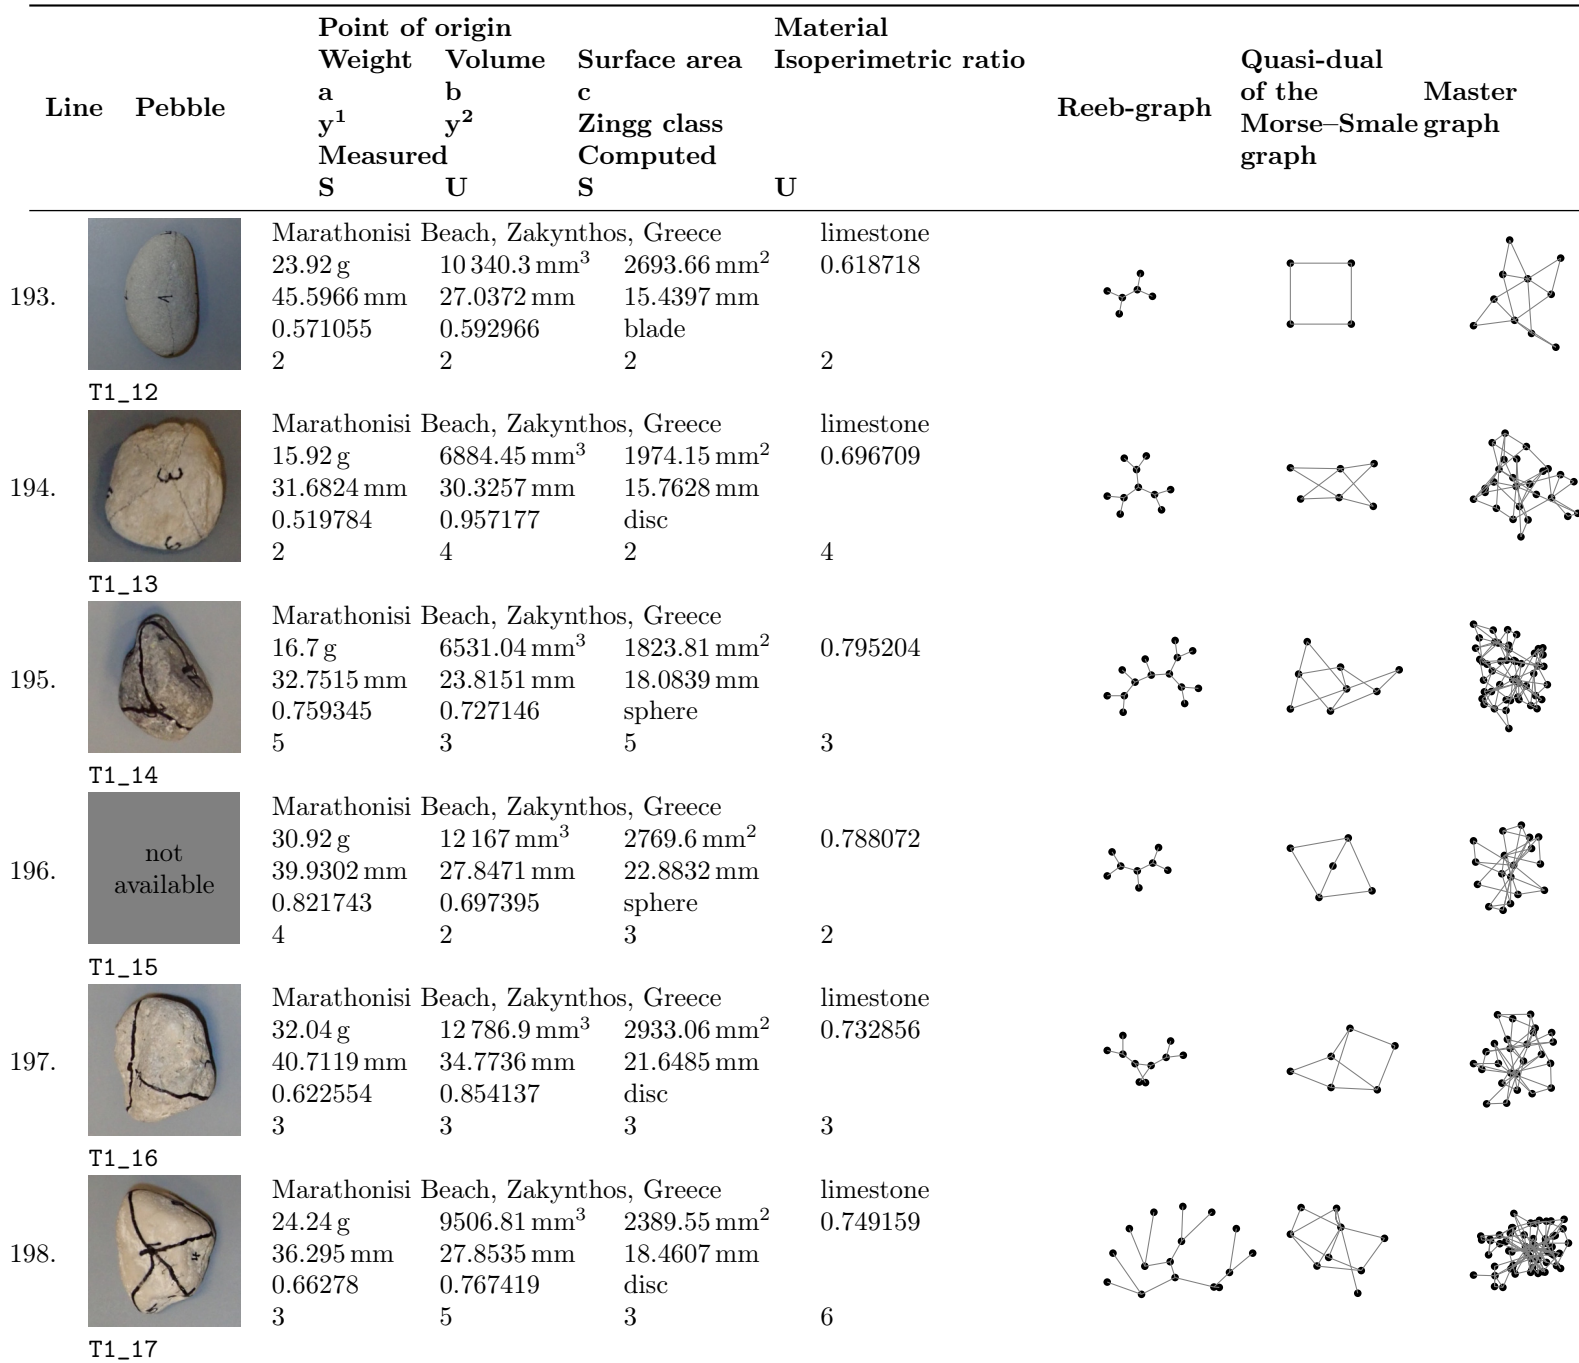  | 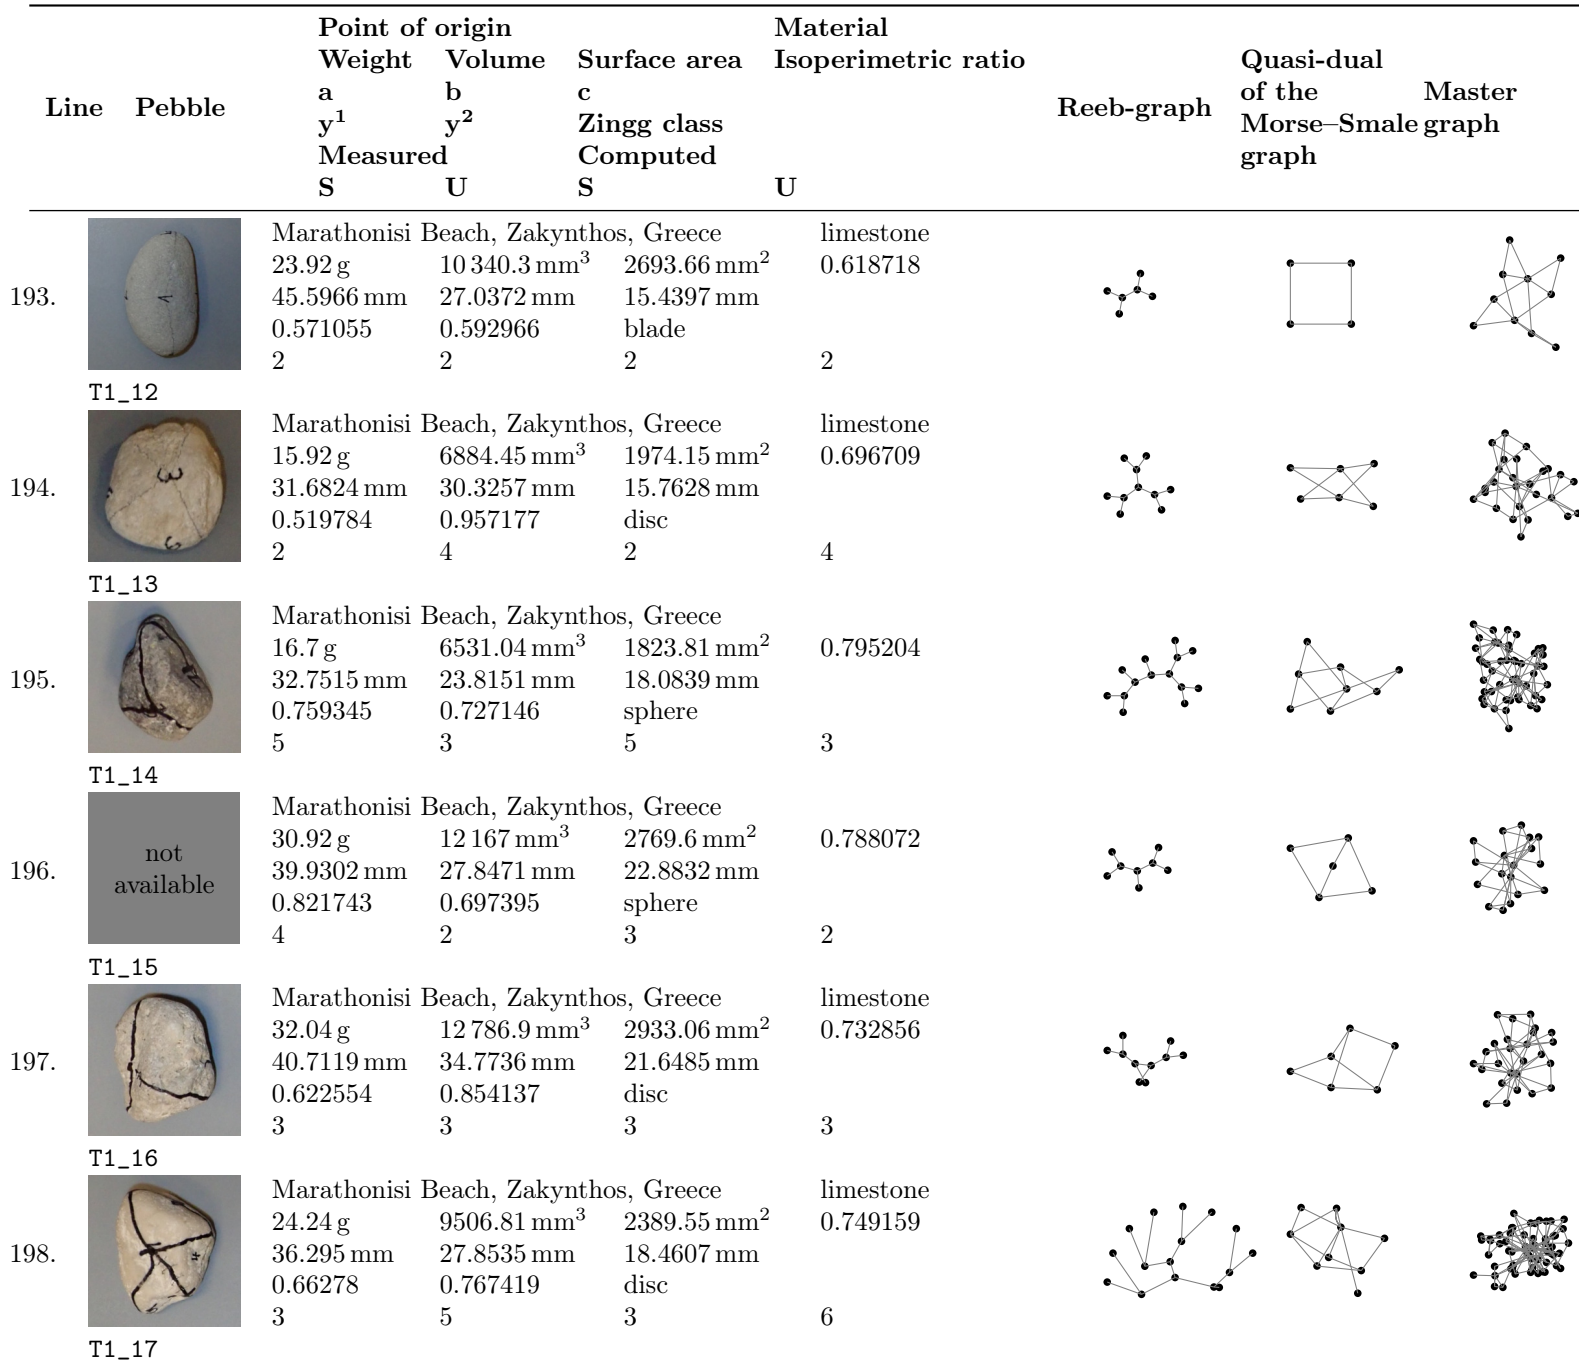  | 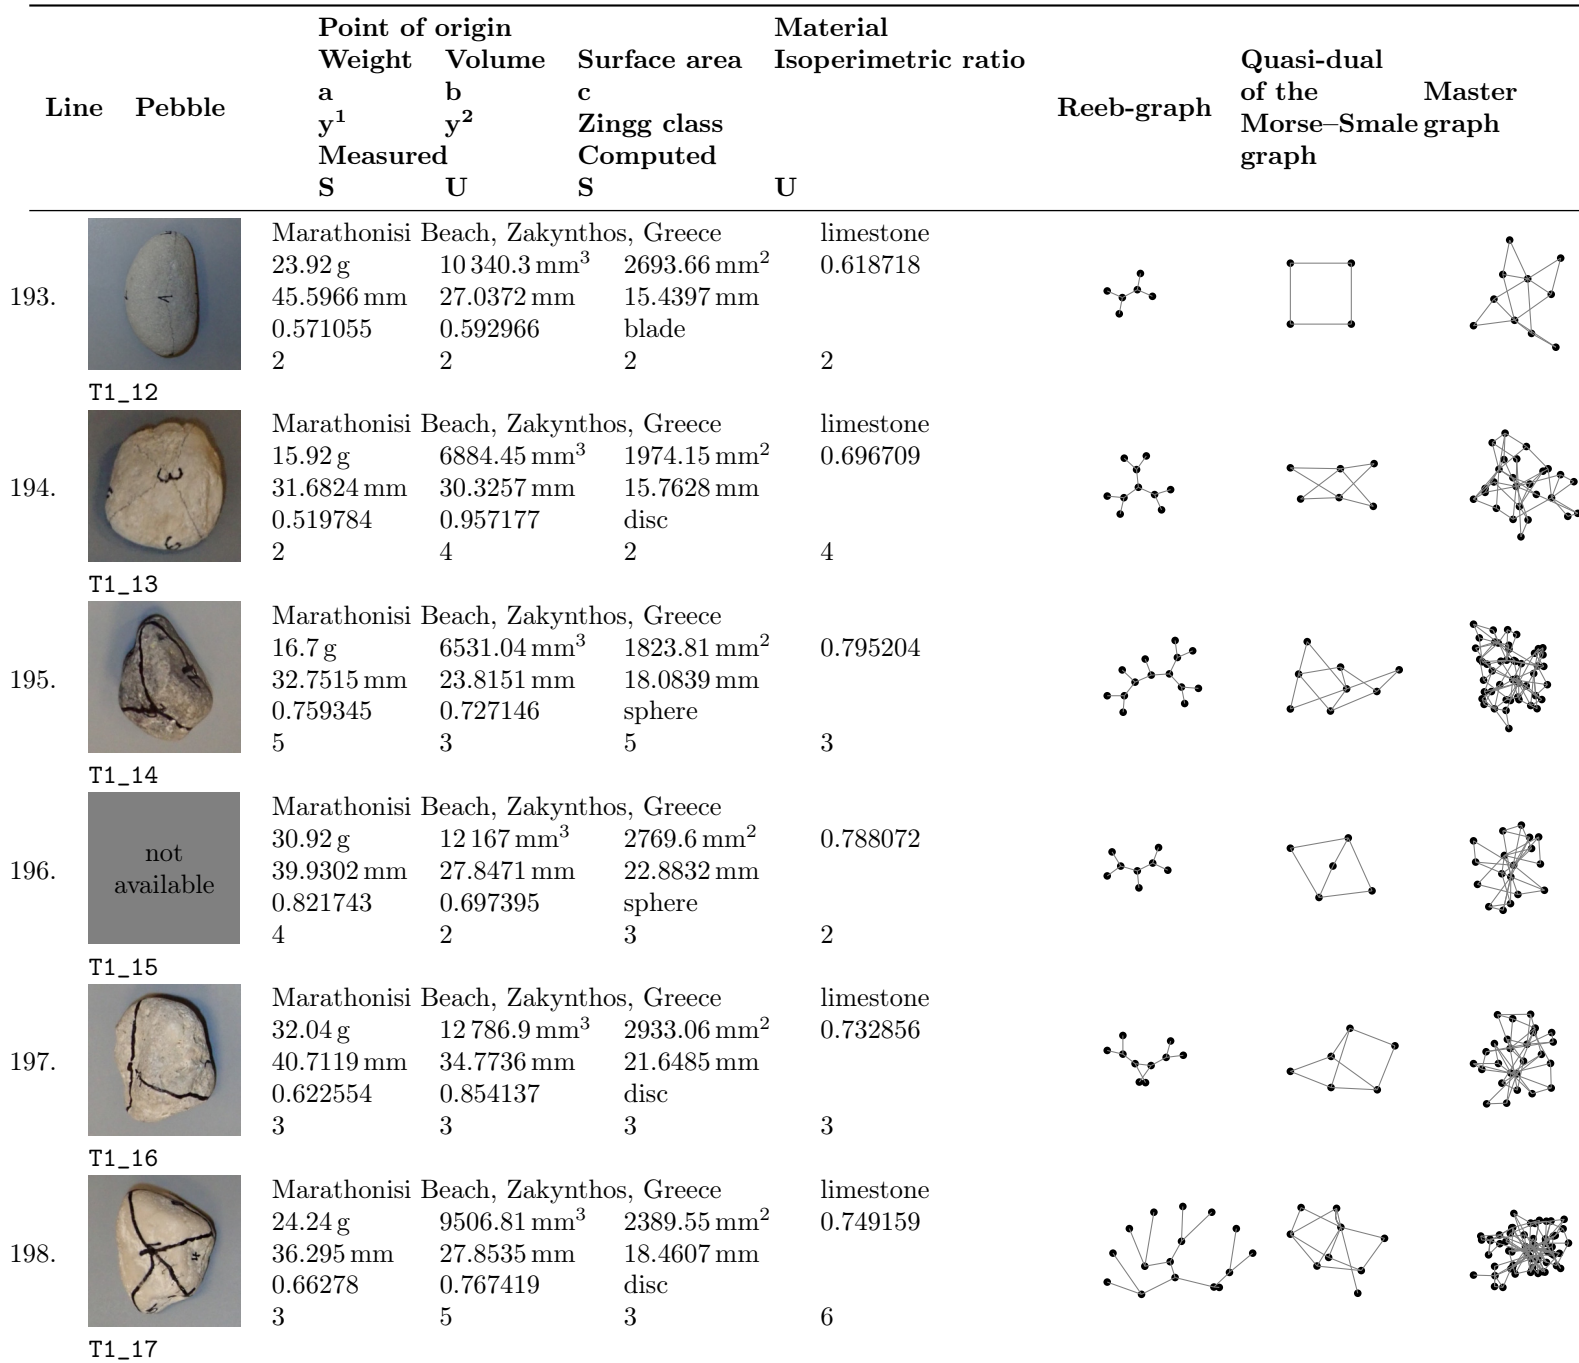  |
|      | T1_15                                                                               |                                                                                |                                                                    |                                                      |                                |                     |                                                                                       |                                                                                       |                                                                                       |
| 197. | 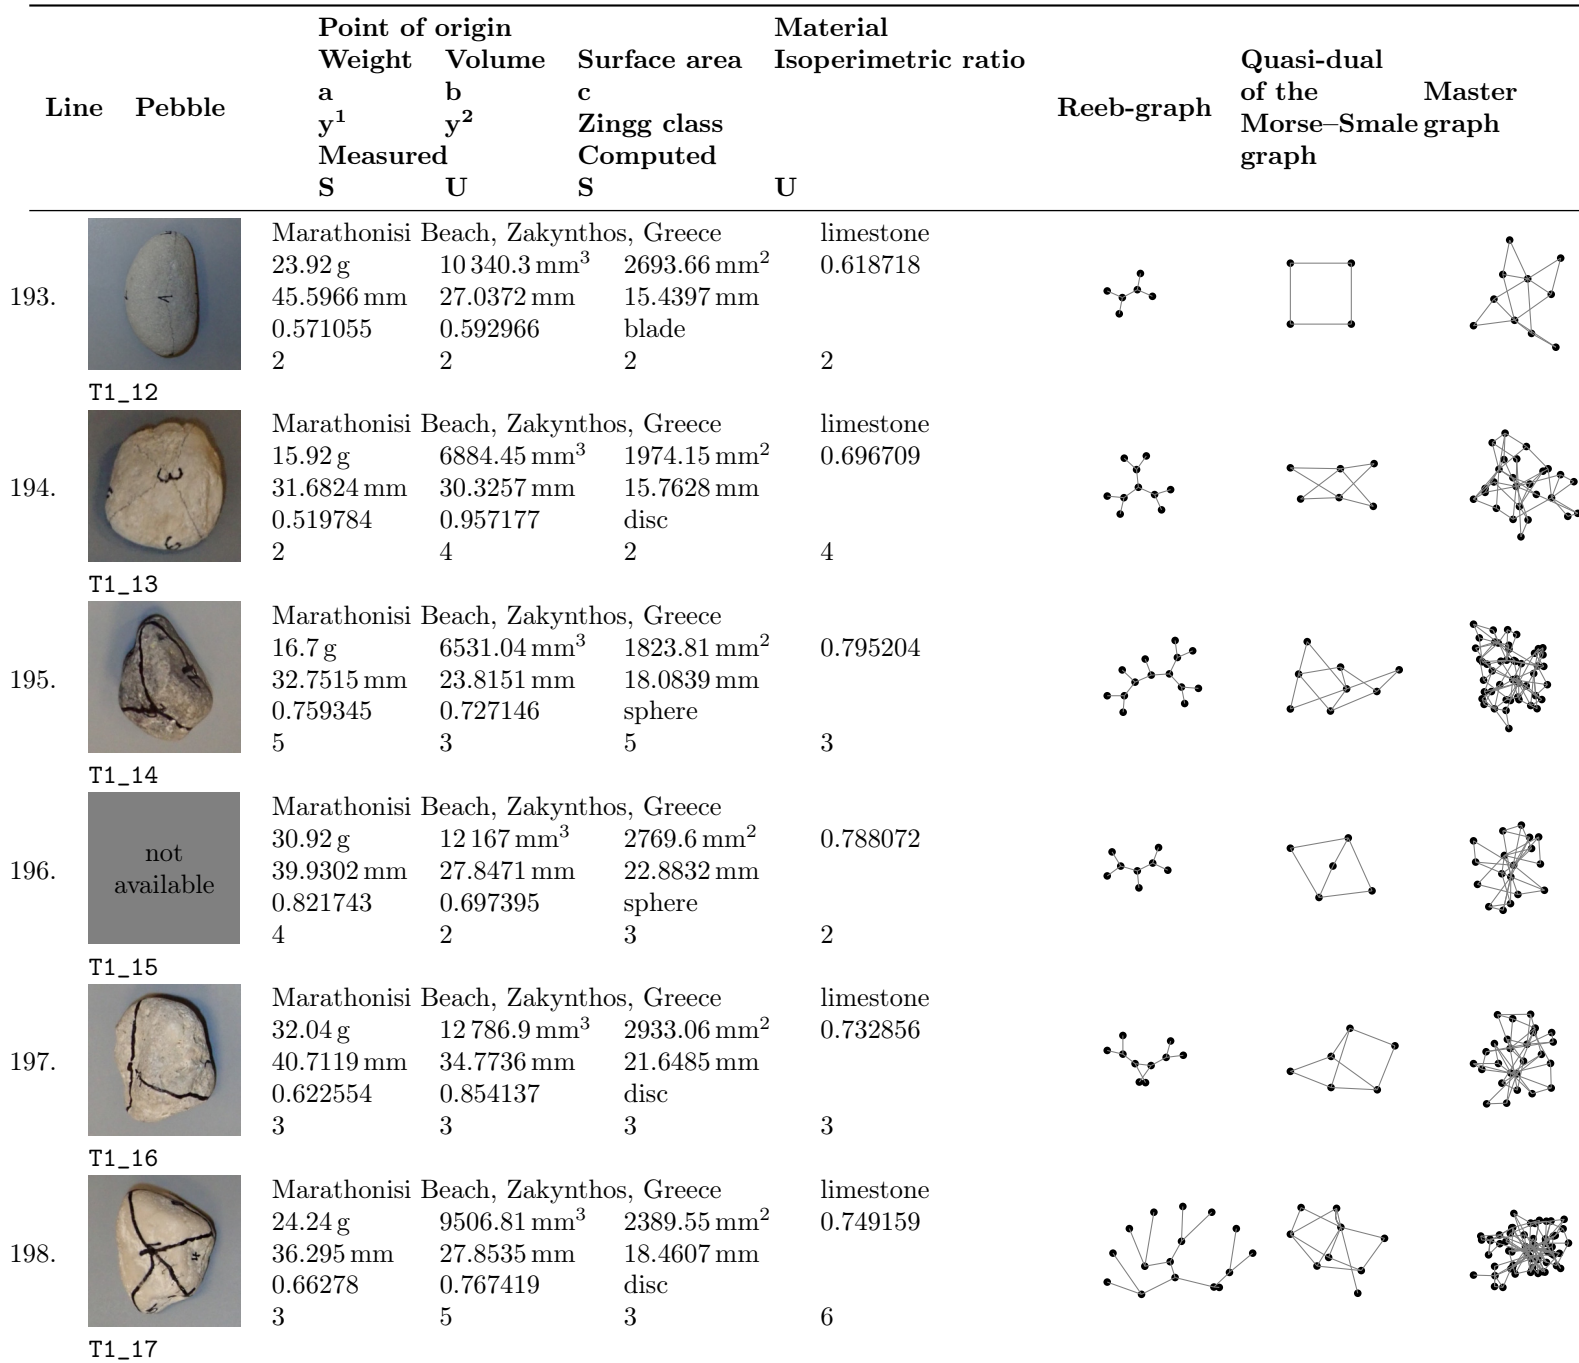 | Marathonisi Beach, Zakynthos, Greece<br>32.04 g<br>40.7119 mm<br>0.622554<br>3 | 32.04 g<br>12 786.9 mm <sup>3</sup><br>34.7736 mm<br>0.854137<br>3 | 2933.06 mm <sup>2</sup><br>21.6485 mm<br>disc<br>3   | limestone<br>0.732856<br><br>3 |                     | 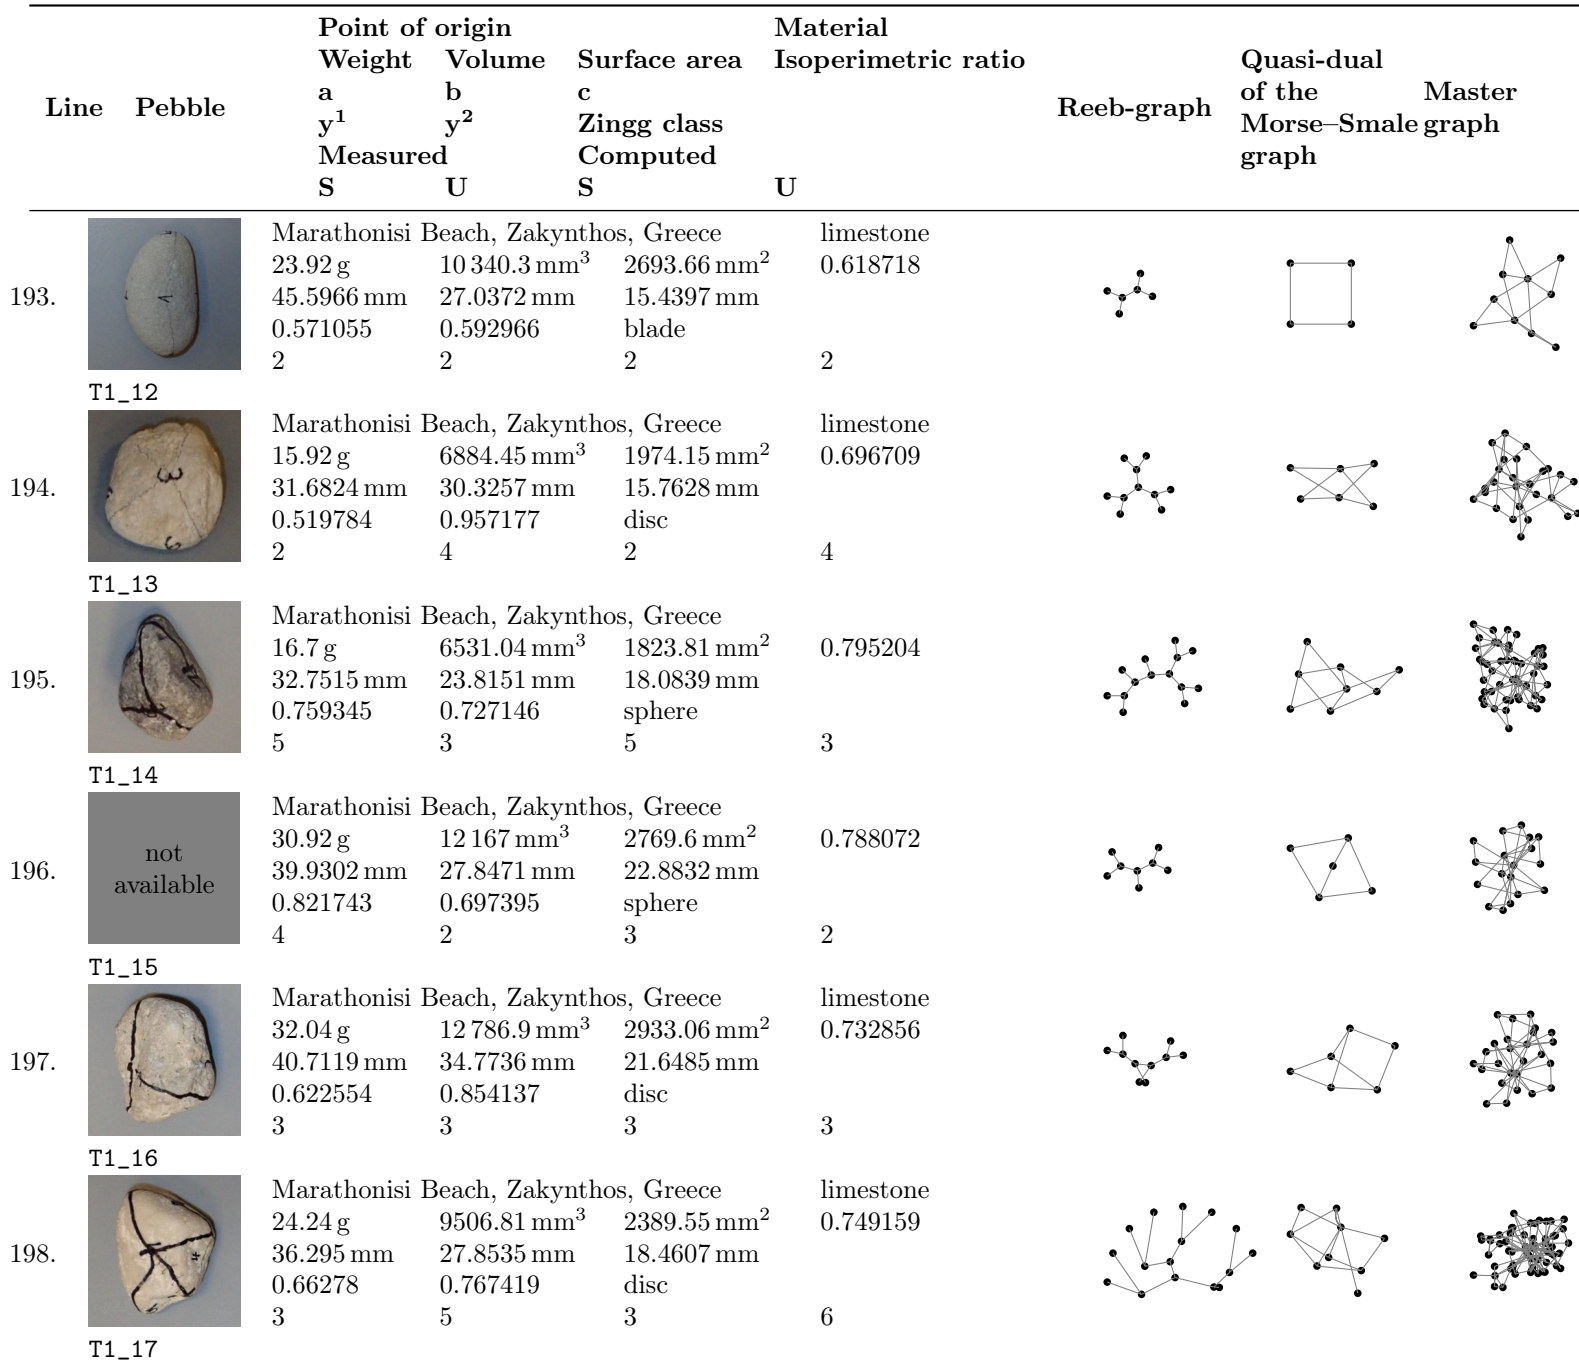 | 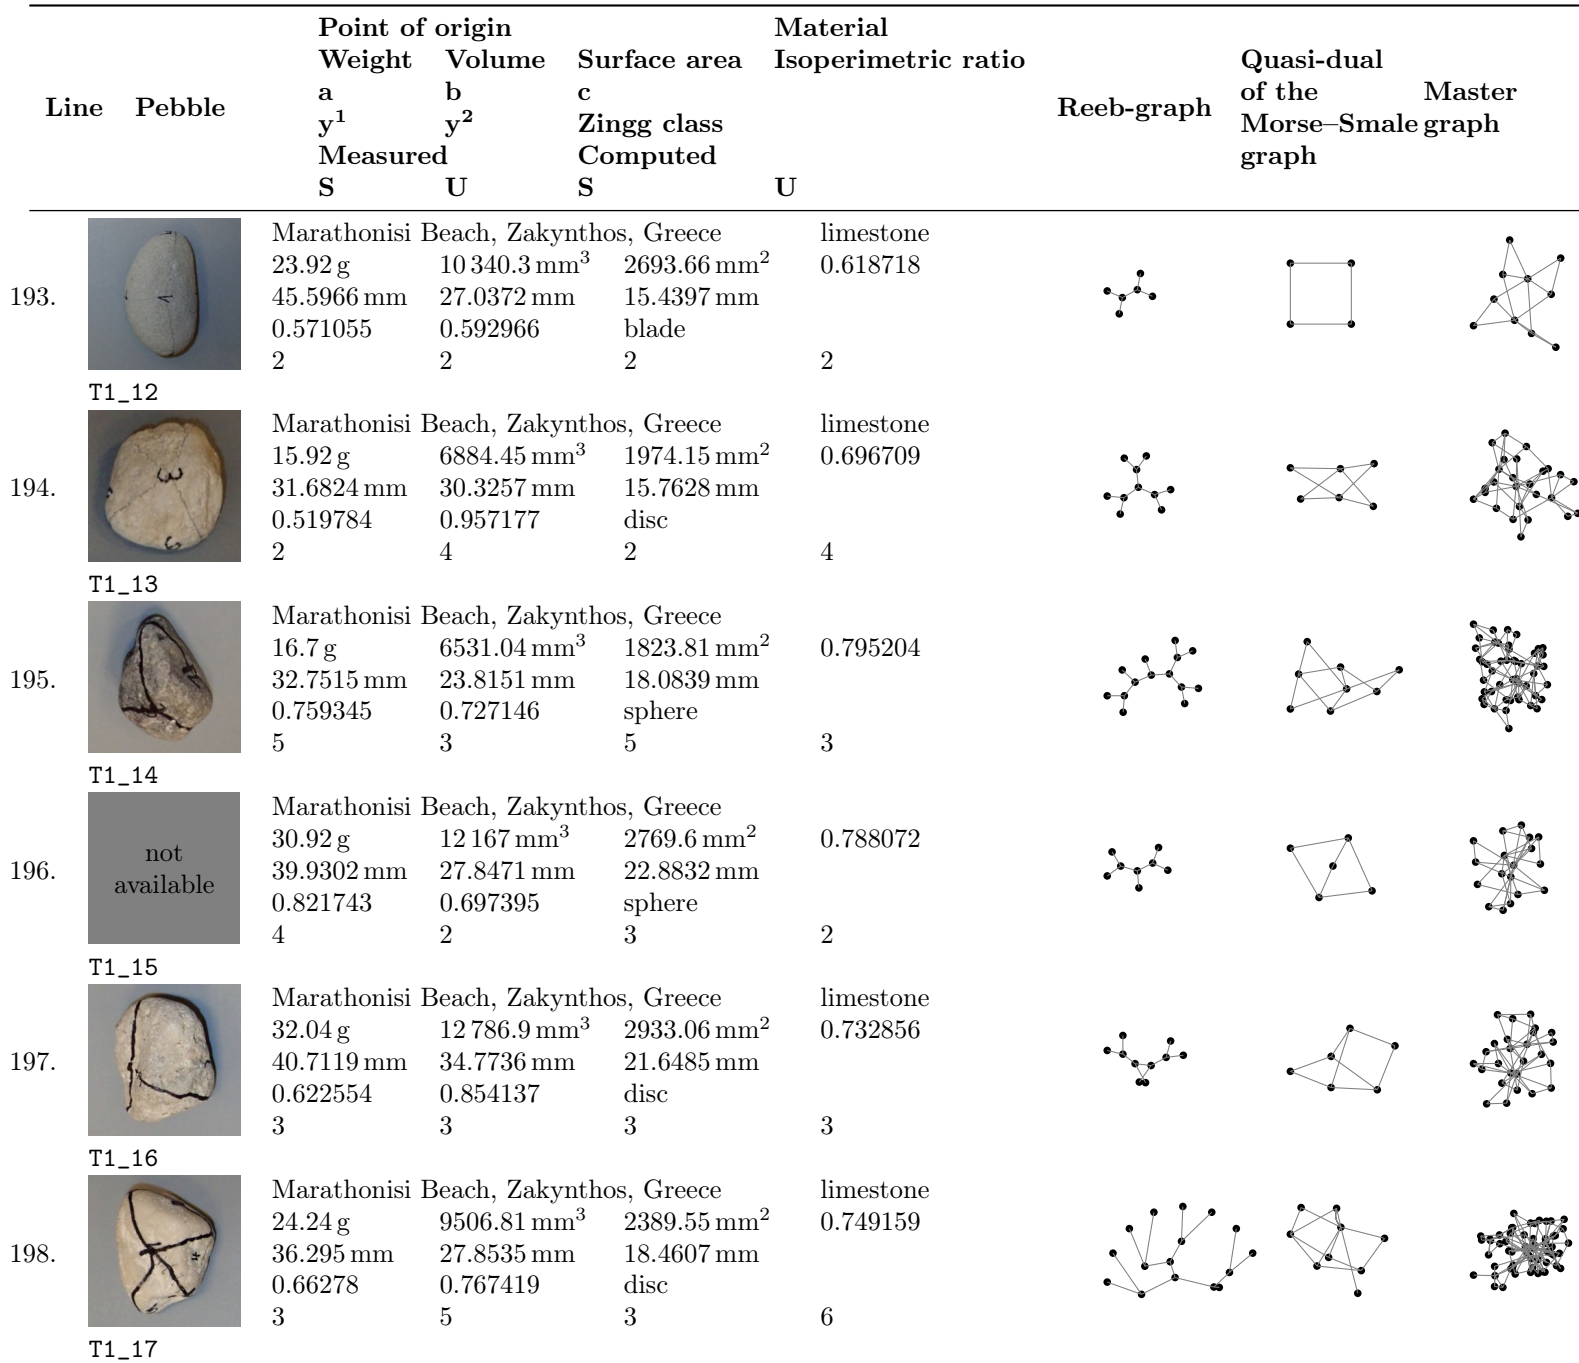 | 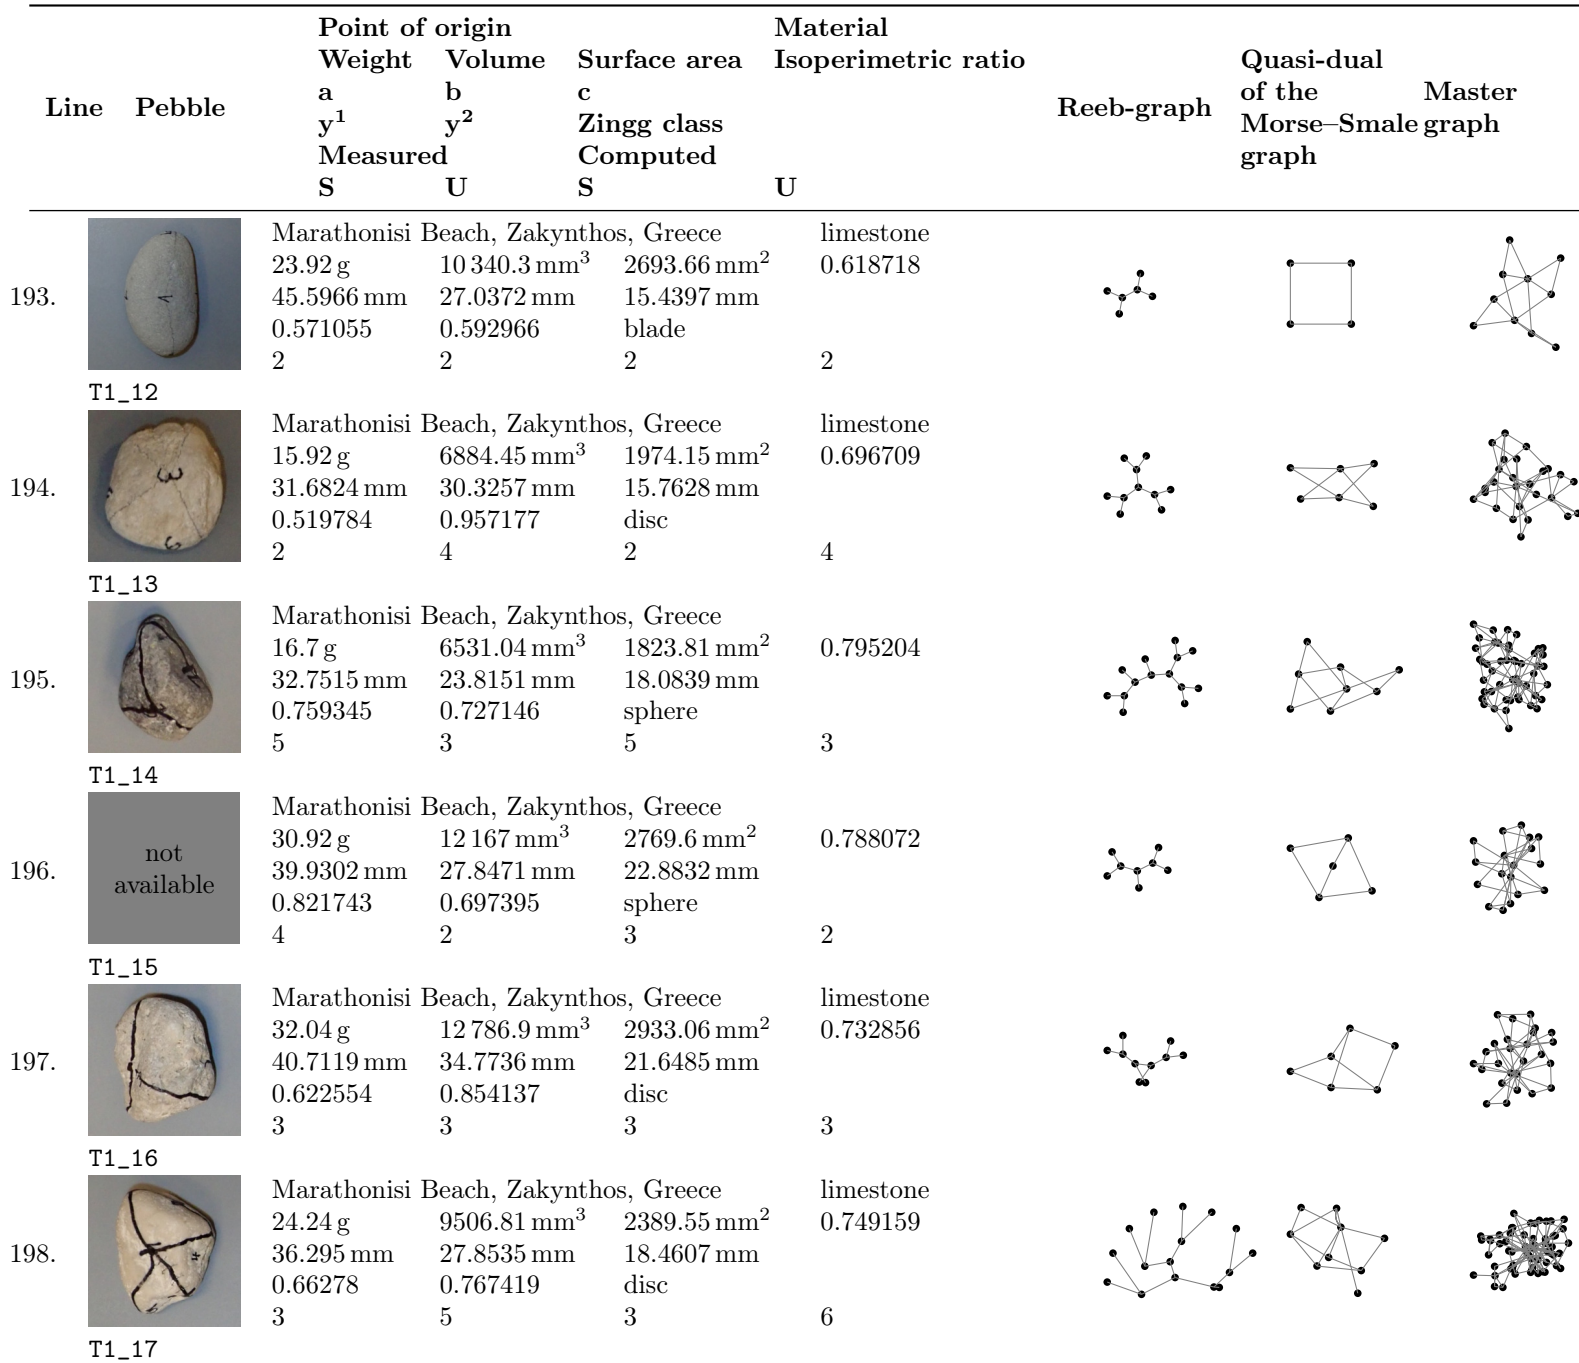 |
|      | T1_16                                                                               |                                                                                |                                                                    |                                                      |                                |                     |                                                                                       |                                                                                       |                                                                                       |
| 198. | 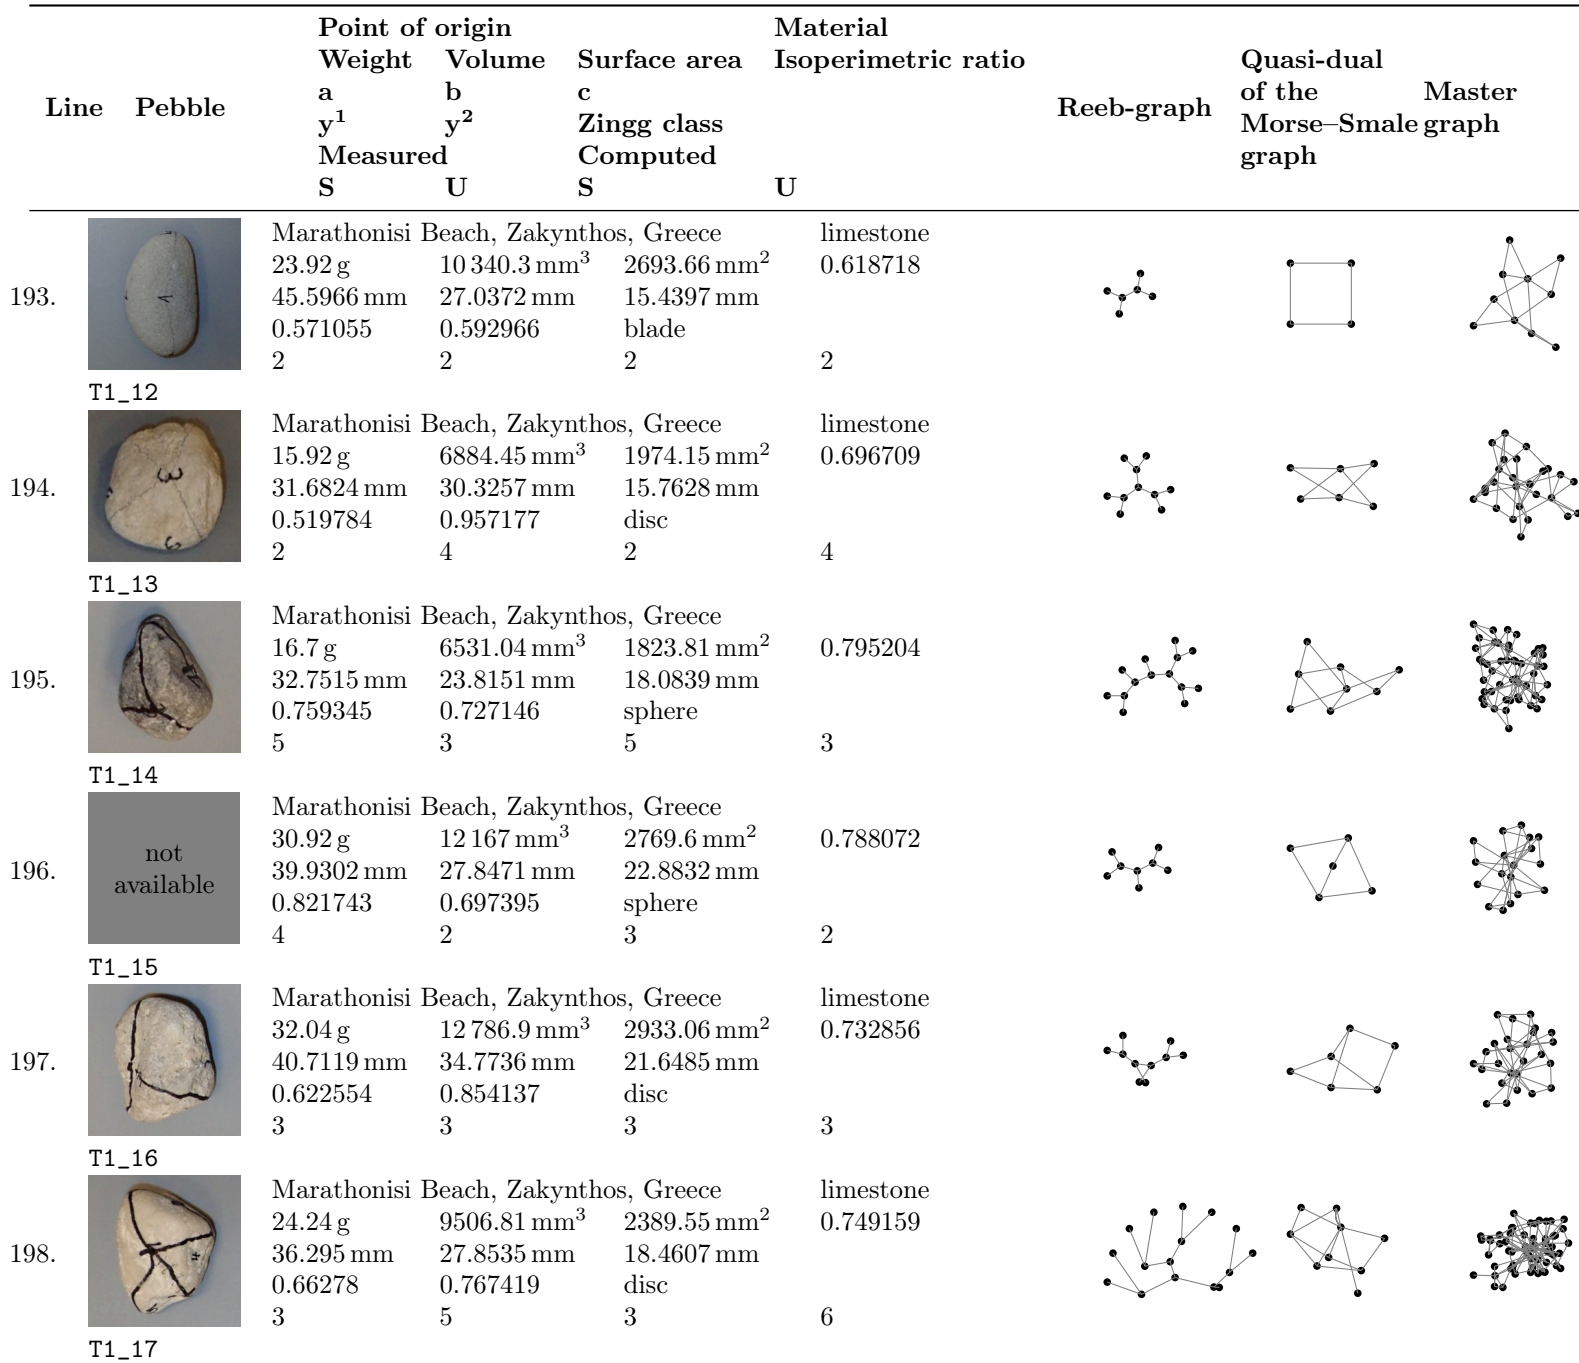 | Marathonisi Beach, Zakynthos, Greece<br>24.24 g<br>36.295 mm<br>0.66278<br>3   | 24.24 g<br>9506.81 mm <sup>3</sup><br>27.8535 mm<br>0.767419<br>5  | 2389.55 mm <sup>2</sup><br>18.4607 mm<br>disc<br>3   | limestone<br>0.749159<br><br>6 |                     | 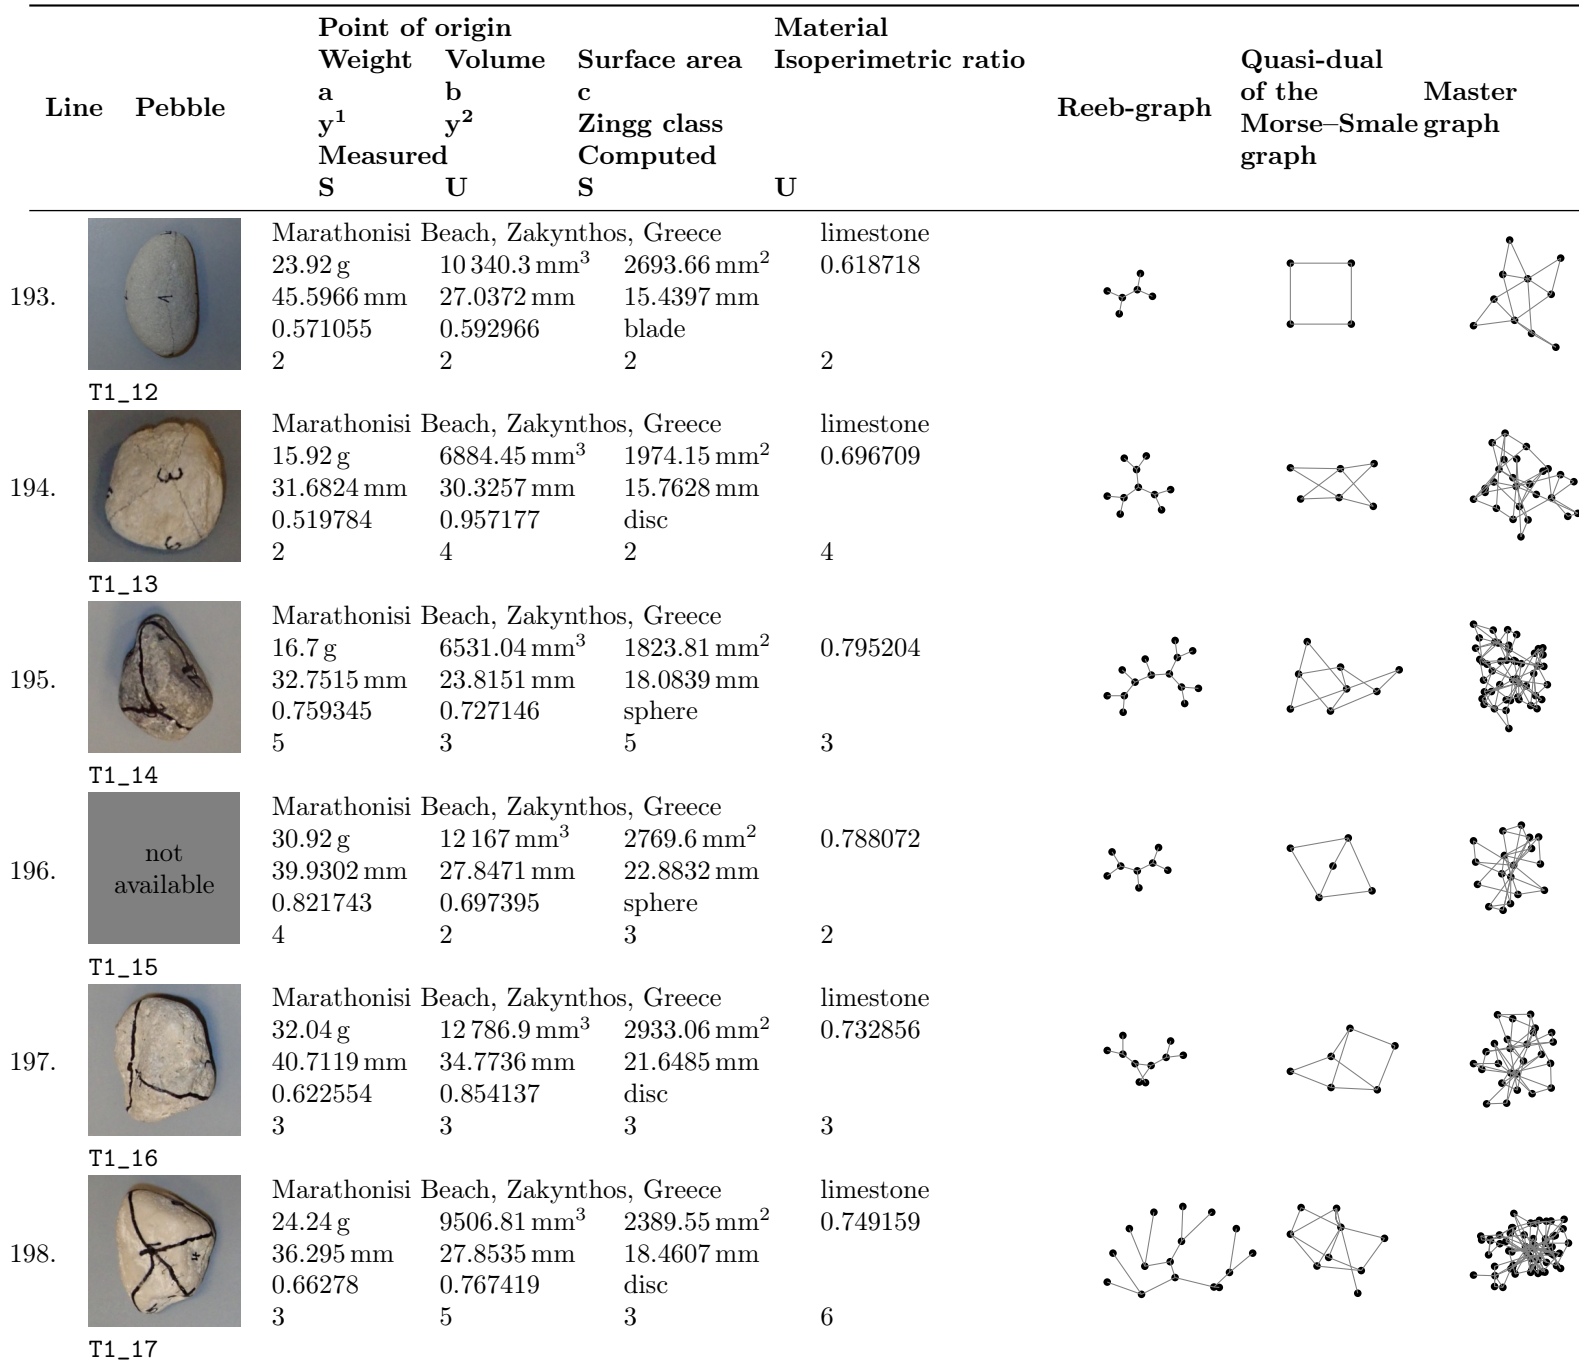 | 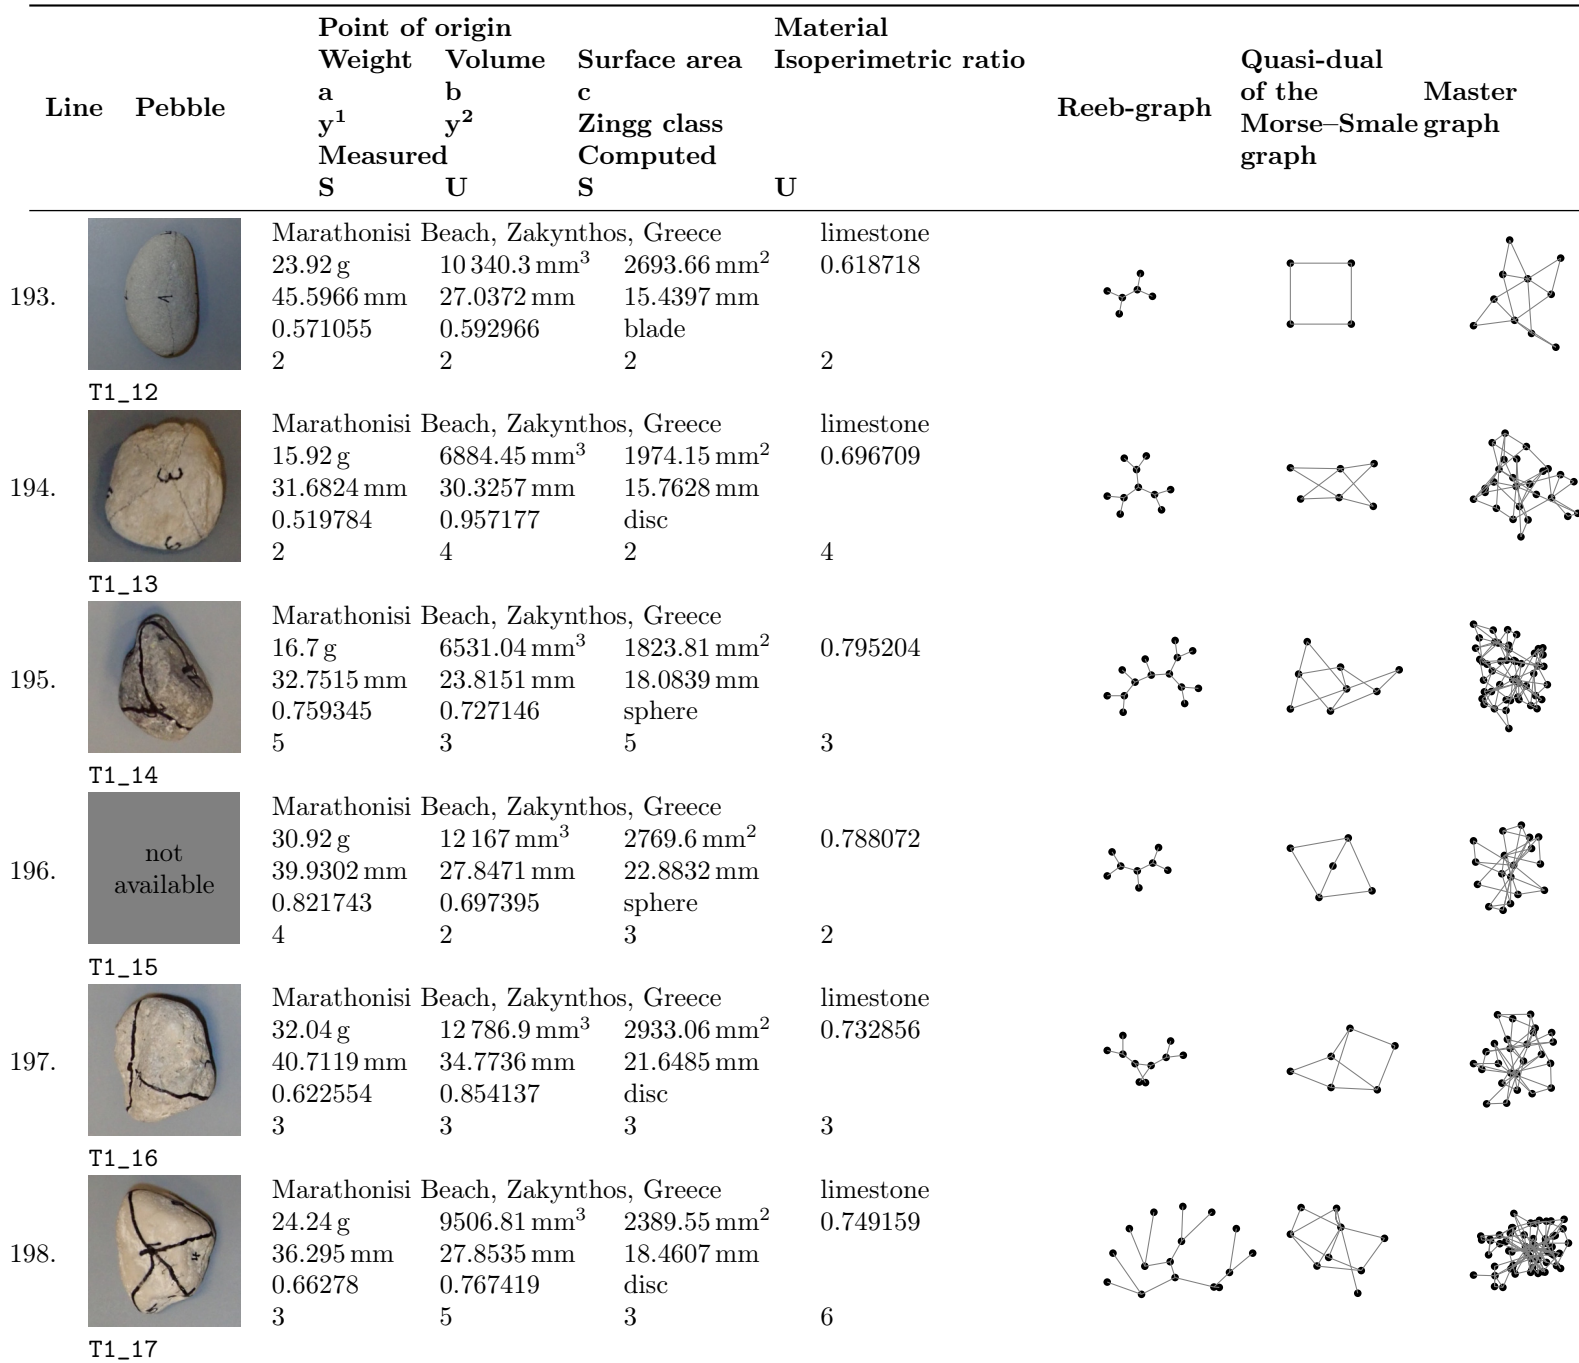 | 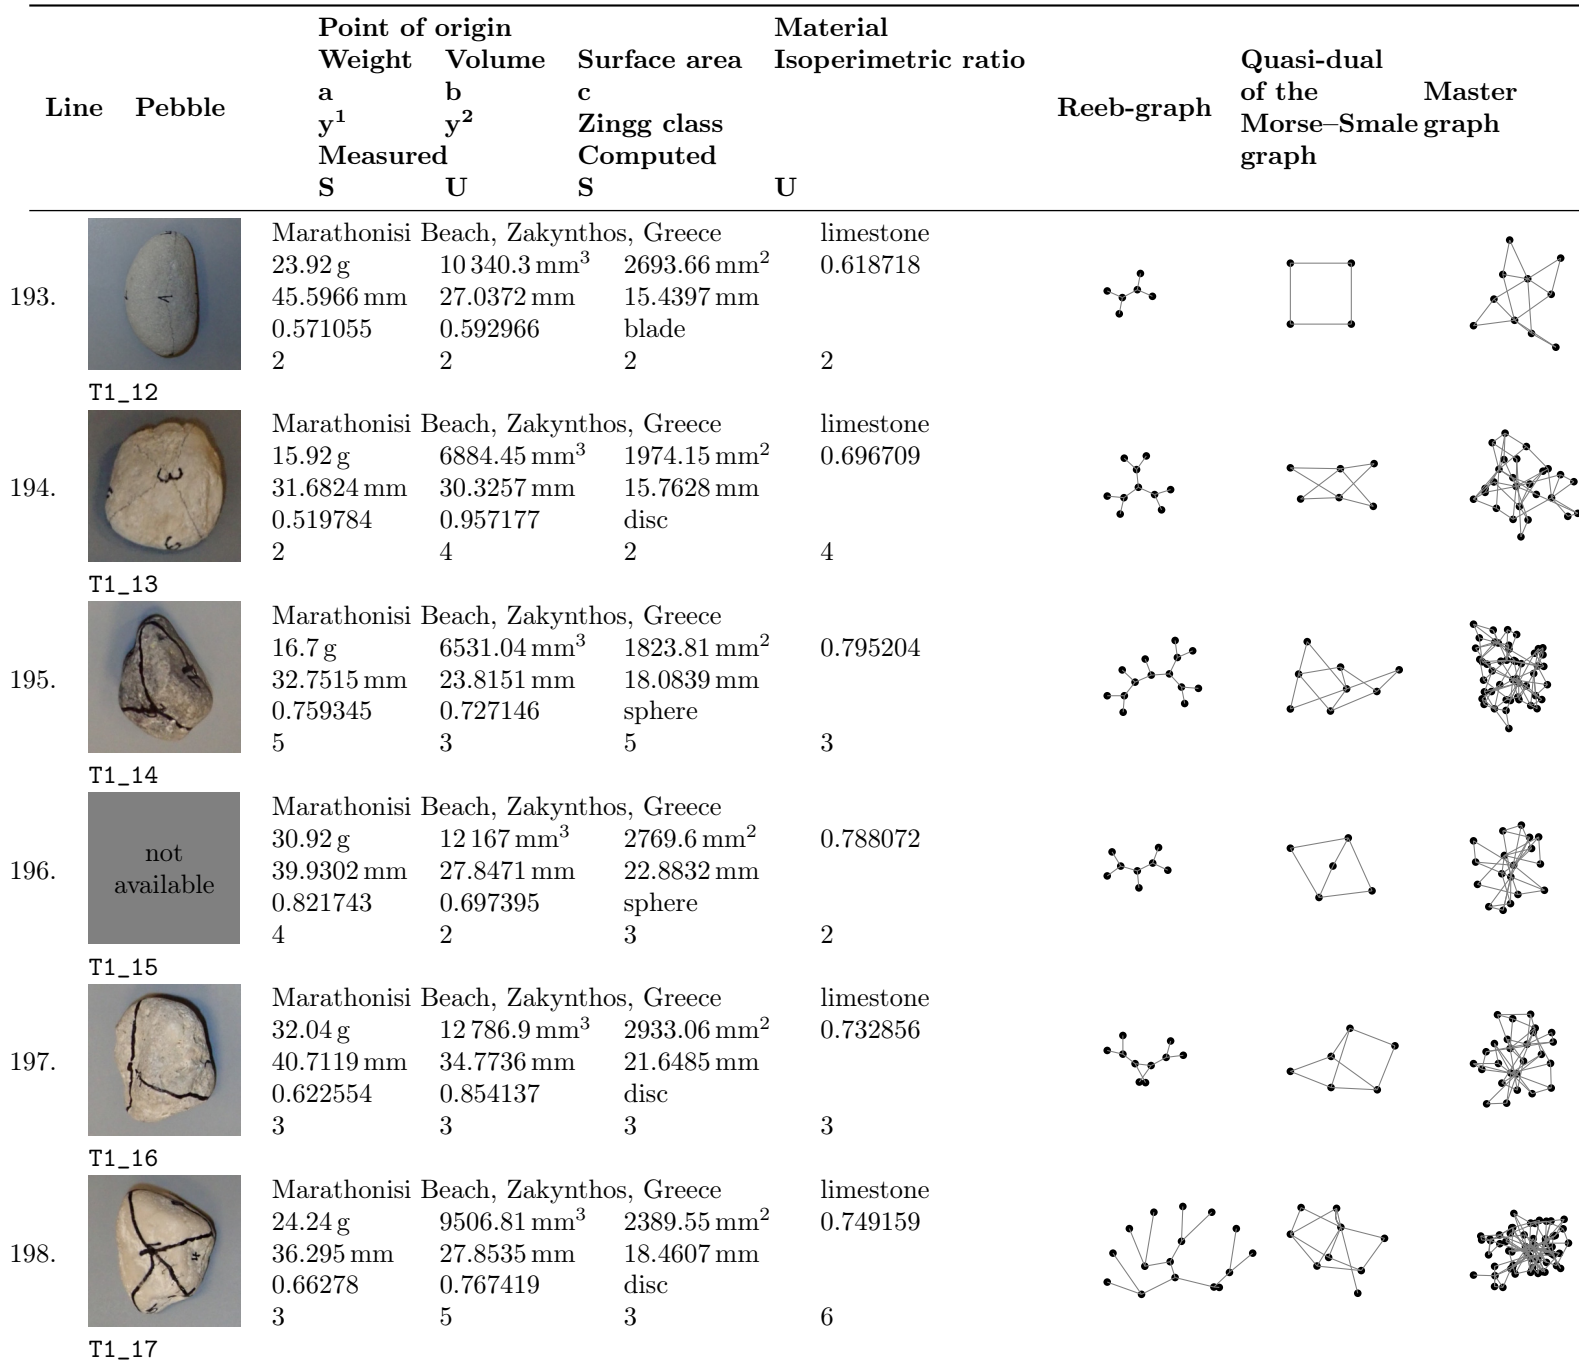 |
|      | T1_17                                                                               |                                                                                |                                                                    |                                                      |                                |                     |                                                                                       |                                                                                       |                                                                                       |

| Line | Pebble                                                                              | Point of origin                                                                |                                                                    | Surface area<br>c<br>Zingg class<br>Computed<br>S    | Material<br>Isoperimetric ratio<br>U | Reeb-graph                                                                            | Quasi-dual<br>of the<br>Morse–Smale<br>graph                                          | Master<br>graph                                                                       |
|------|-------------------------------------------------------------------------------------|--------------------------------------------------------------------------------|--------------------------------------------------------------------|------------------------------------------------------|--------------------------------------|---------------------------------------------------------------------------------------|---------------------------------------------------------------------------------------|---------------------------------------------------------------------------------------|
|      |                                                                                     | Weight                                                                         | Volume                                                             |                                                      |                                      |                                                                                       |                                                                                       |                                                                                       |
|      |                                                                                     | a<br>y <sup>1</sup><br>Measured<br>S                                           | b<br>y <sup>2</sup><br>U                                           |                                                      |                                      |                                                                                       |                                                                                       |                                                                                       |
|      |                                                                                     |                                                                                |                                                                    |                                                      |                                      |                                                                                       |                                                                                       |                                                                                       |
| 199. | 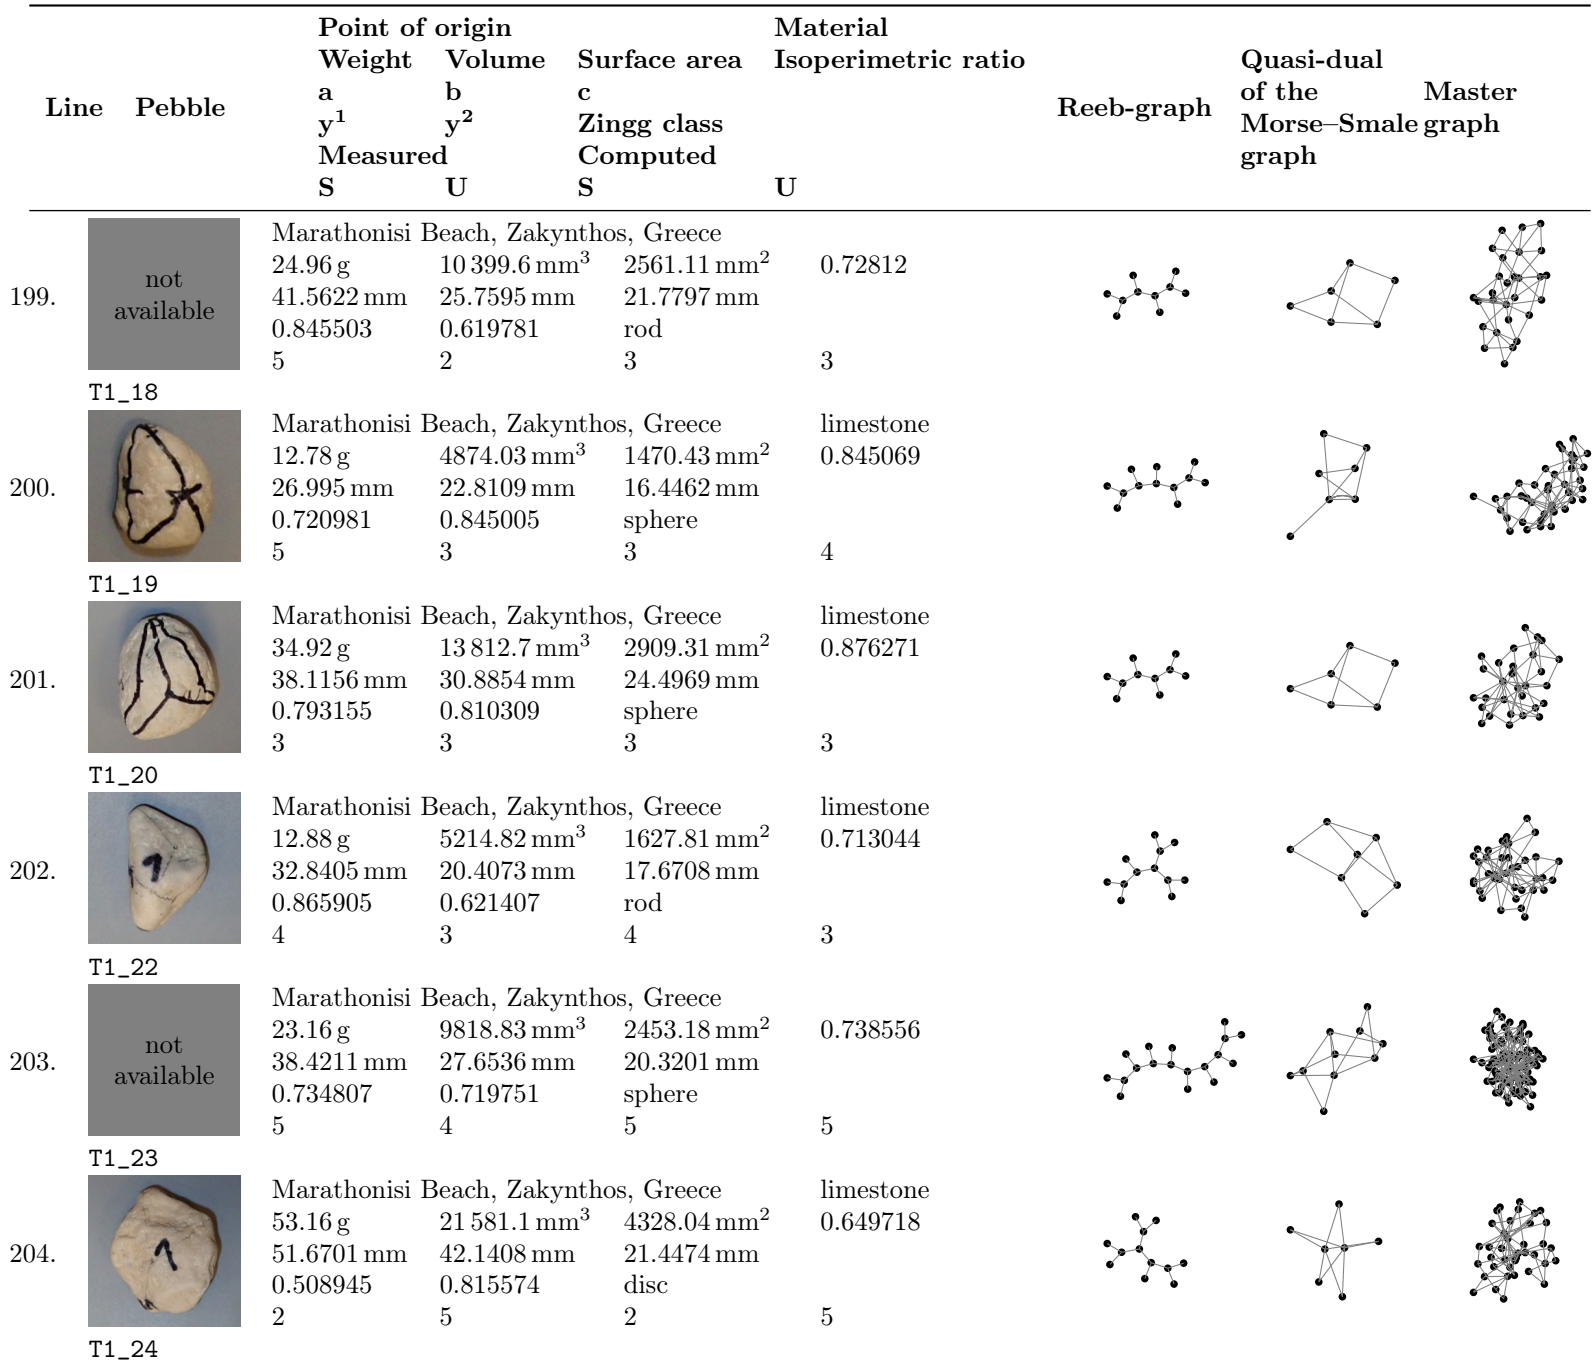   | Marathonisi Beach, Zakynthos, Greece<br>24.96 g<br>41.5622 mm<br>0.845503<br>5 | 24.96 g<br>10 399.6 mm <sup>3</sup><br>25.7595 mm<br>0.619781<br>2 | 2561.11 mm <sup>2</sup><br>21.7797 mm<br>rod<br>3    | 0.72812<br><br><br>3                 | 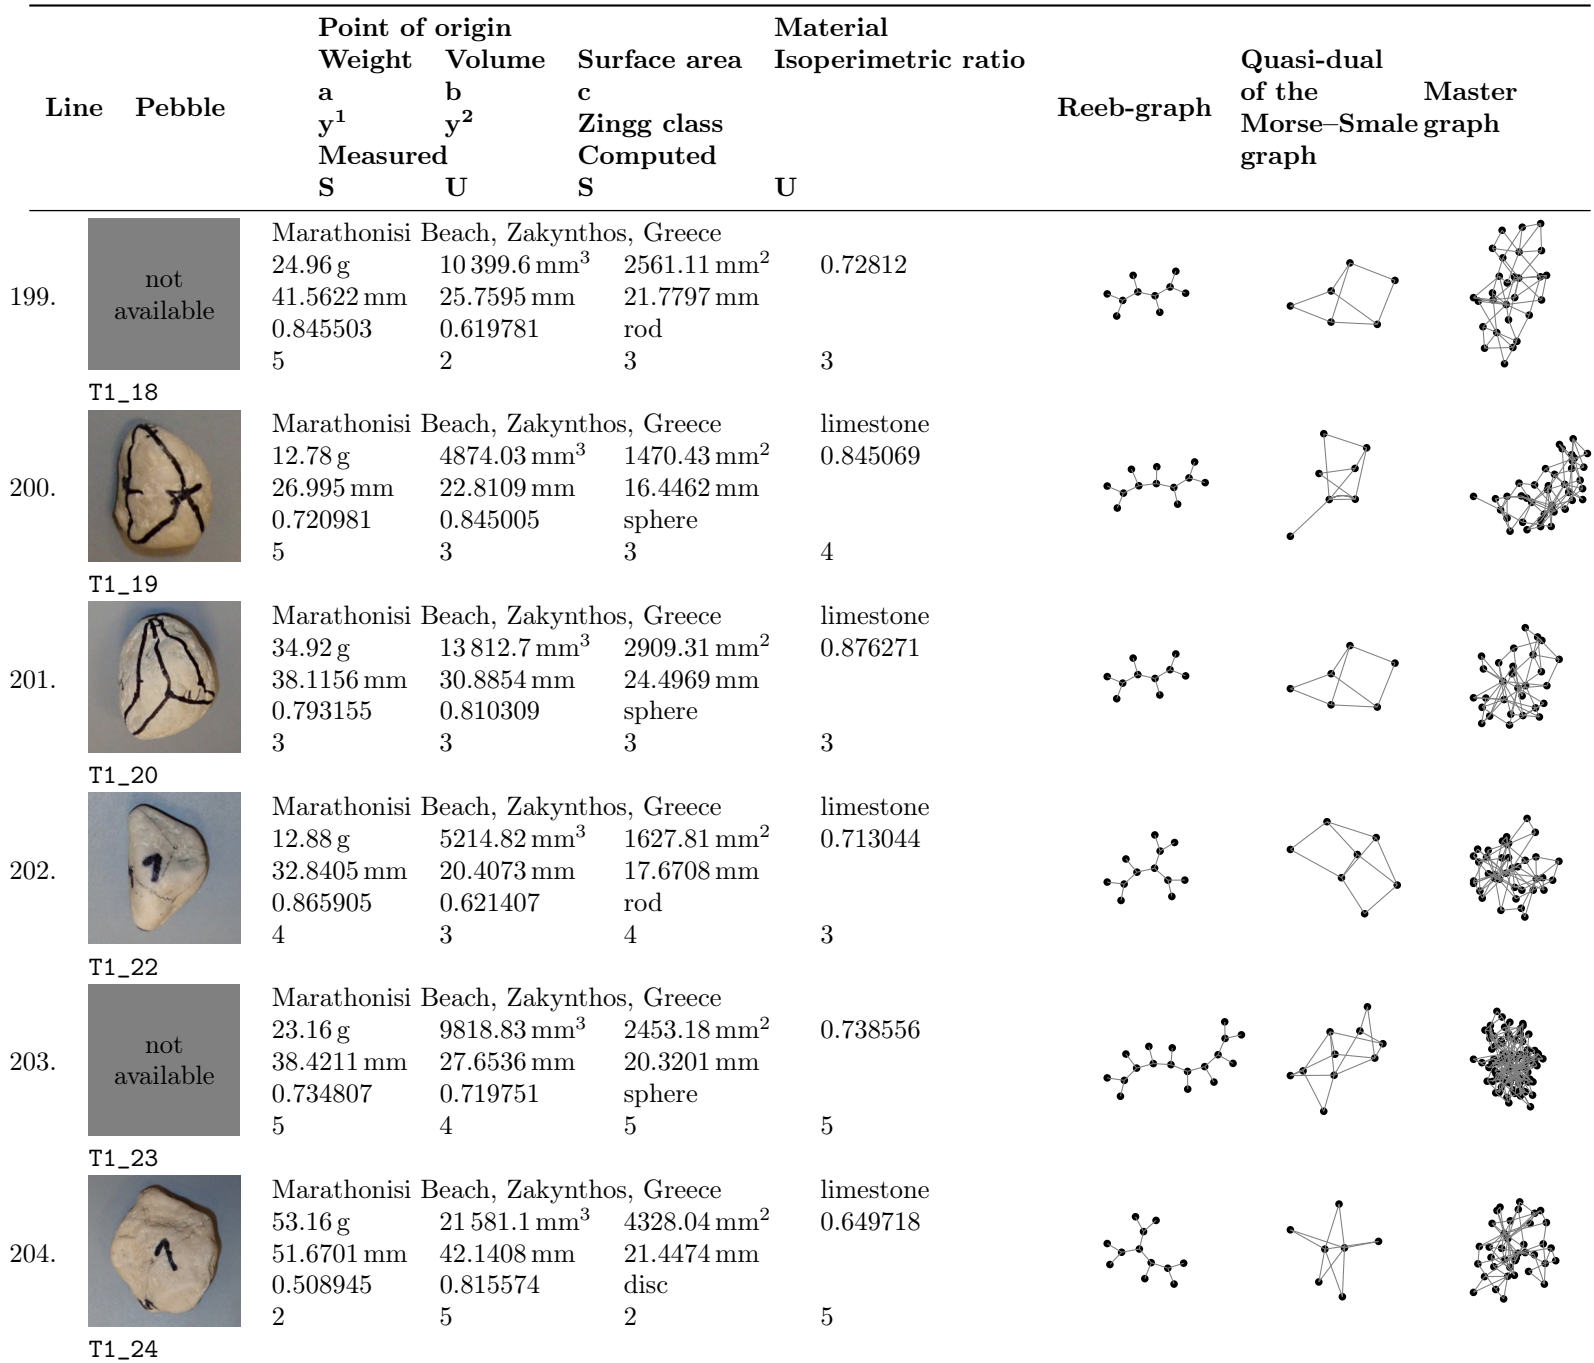   | 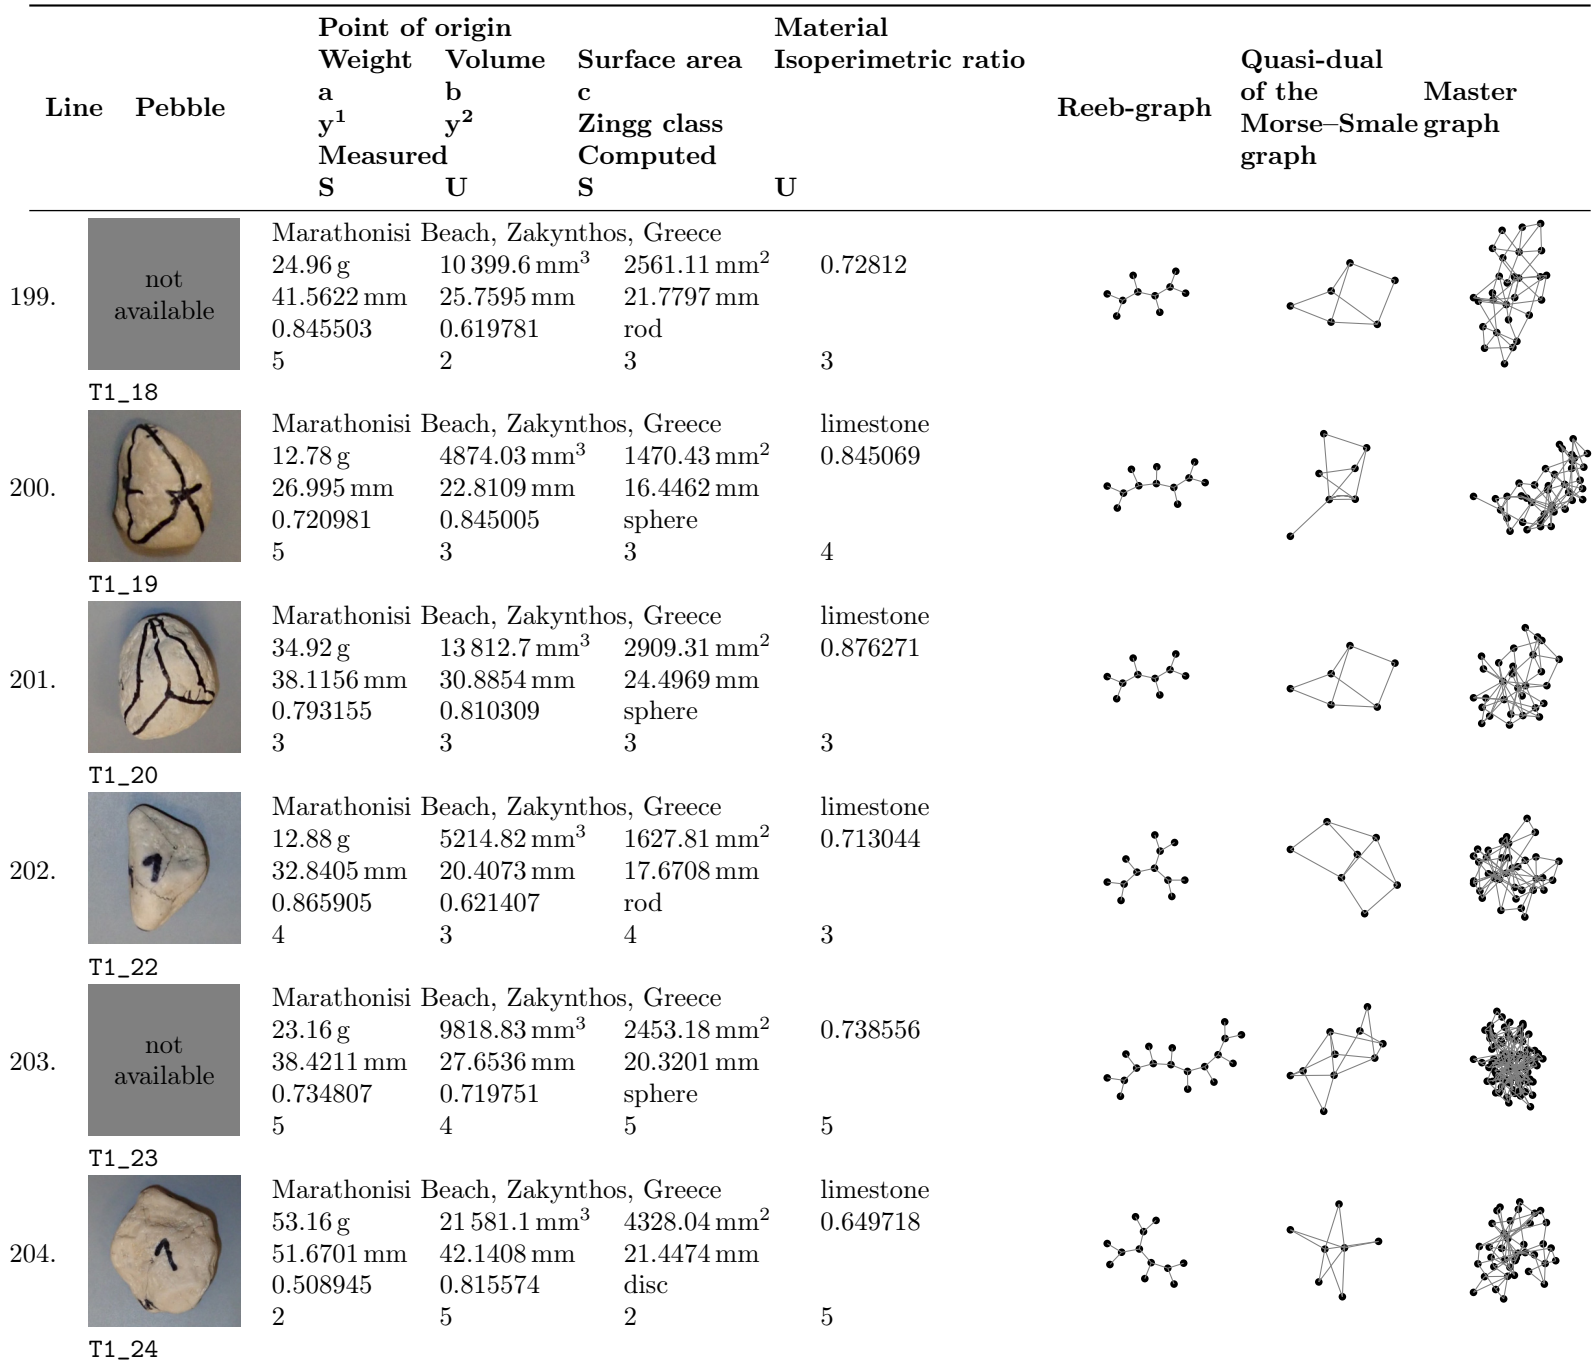   | 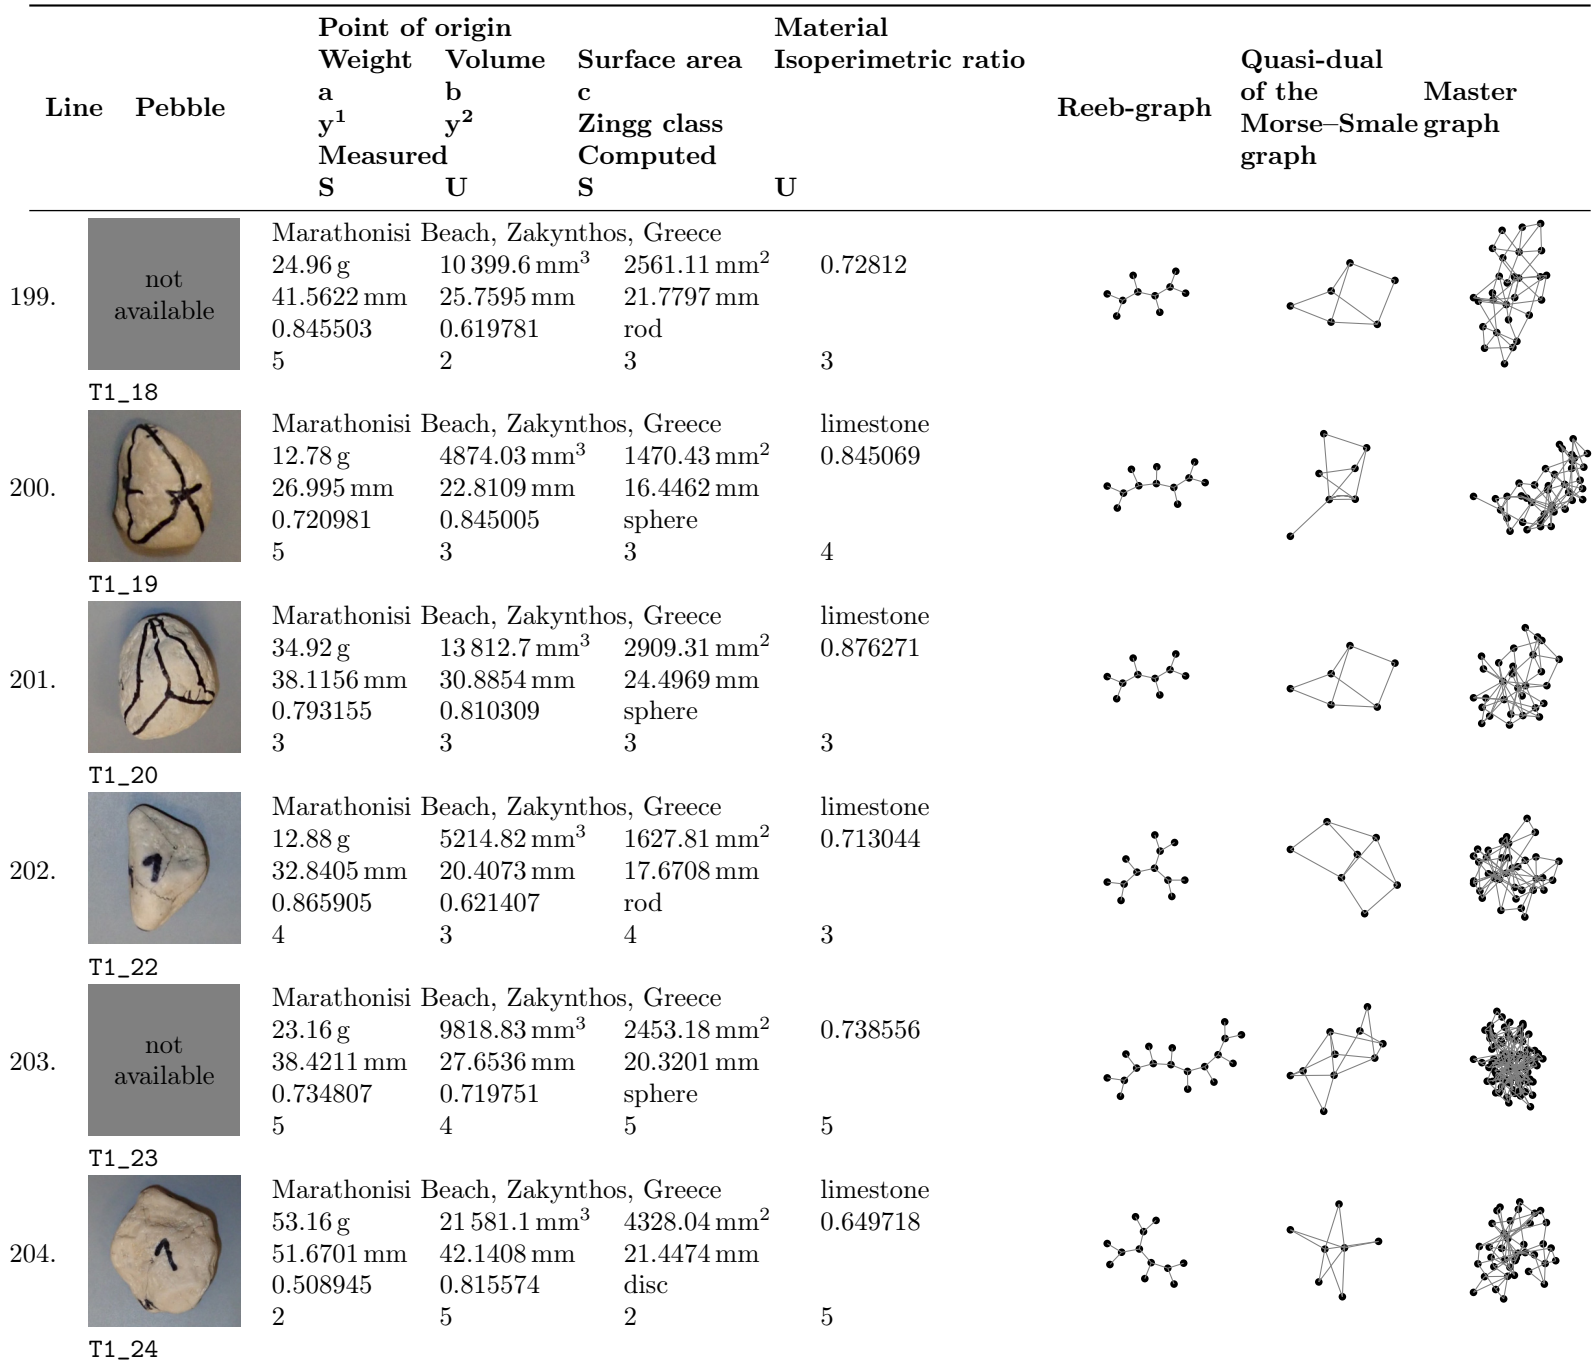   |
|      | T1_18                                                                               |                                                                                |                                                                    |                                                      |                                      |                                                                                       |                                                                                       |                                                                                       |
| 200. | 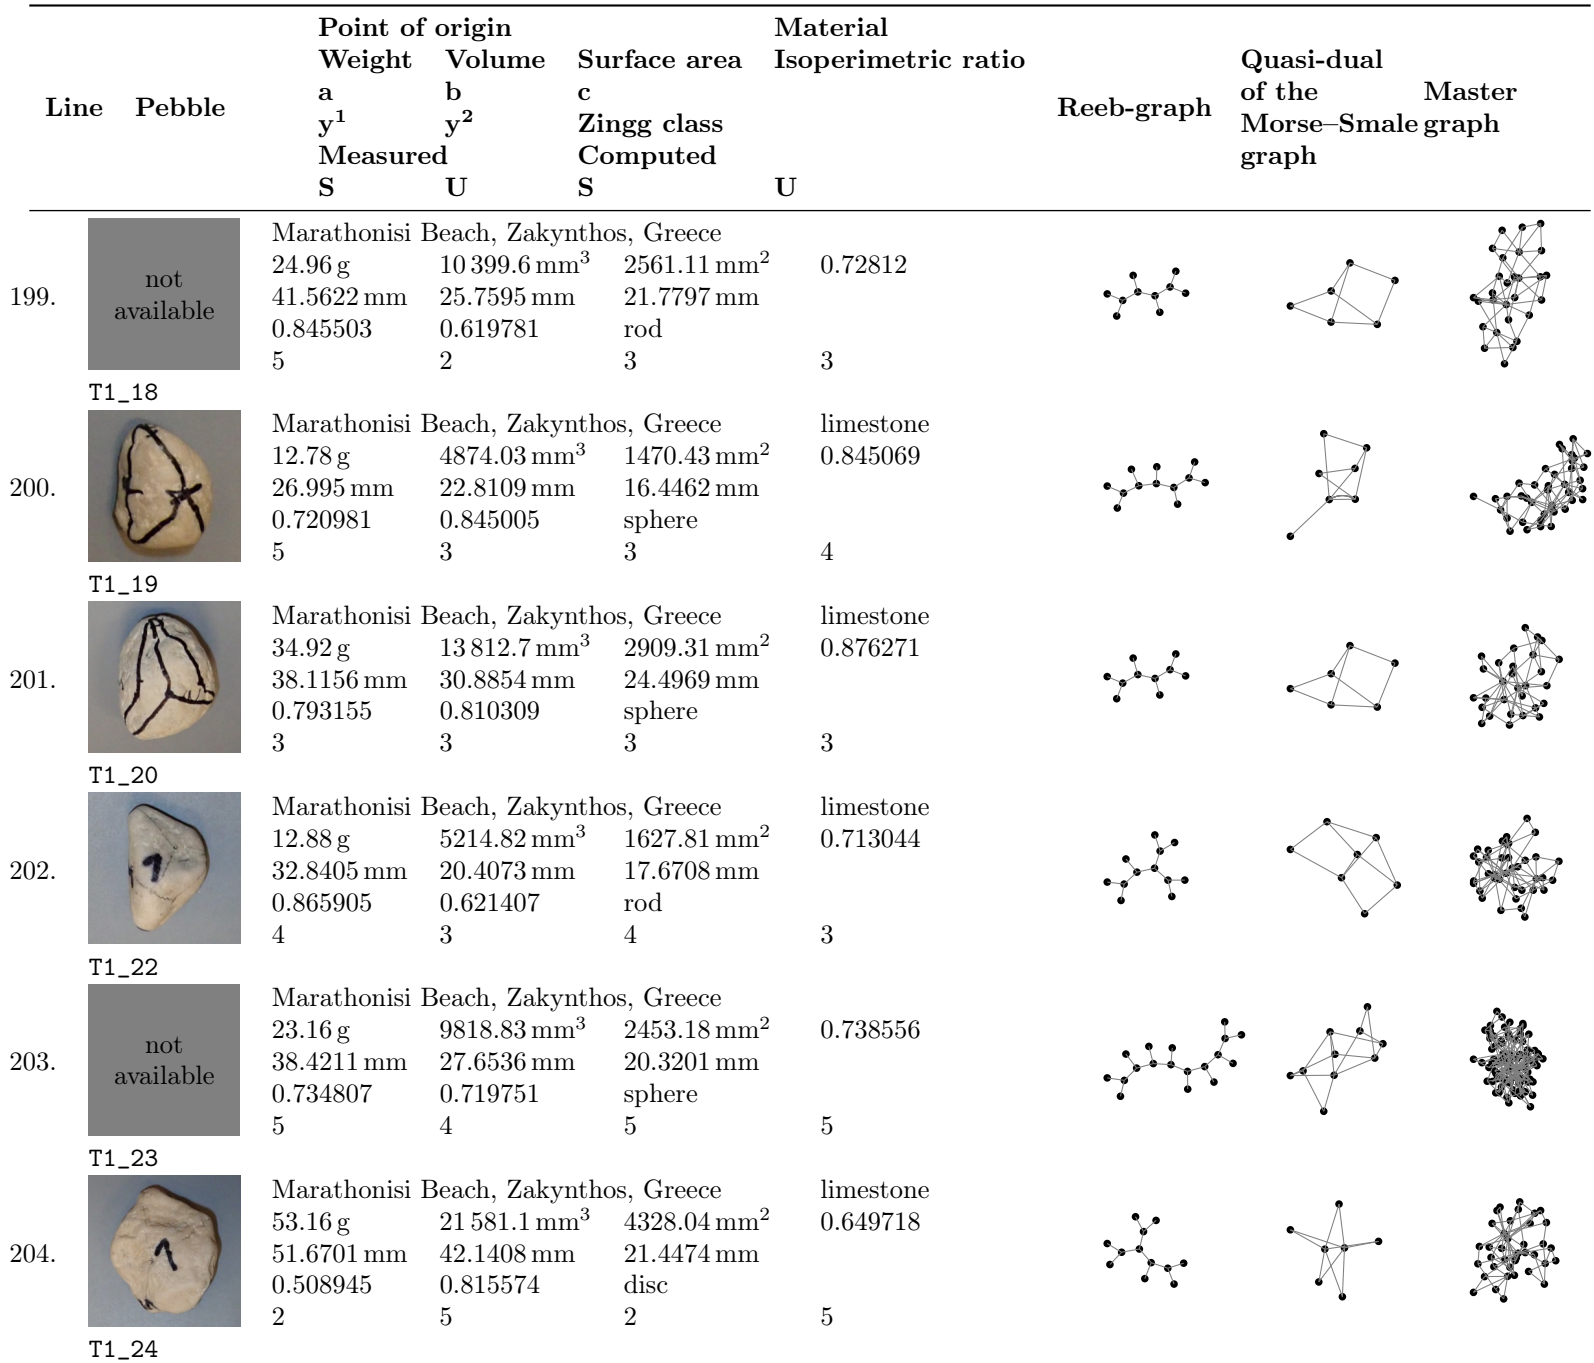   | Marathonisi Beach, Zakynthos, Greece<br>12.78 g<br>26.995 mm<br>0.720981<br>5  | 12.78 g<br>4874.03 mm <sup>3</sup><br>22.8109 mm<br>0.845005<br>3  | 1470.43 mm <sup>2</sup><br>16.4462 mm<br>sphere<br>3 | limestone<br>0.845069<br><br>4       | 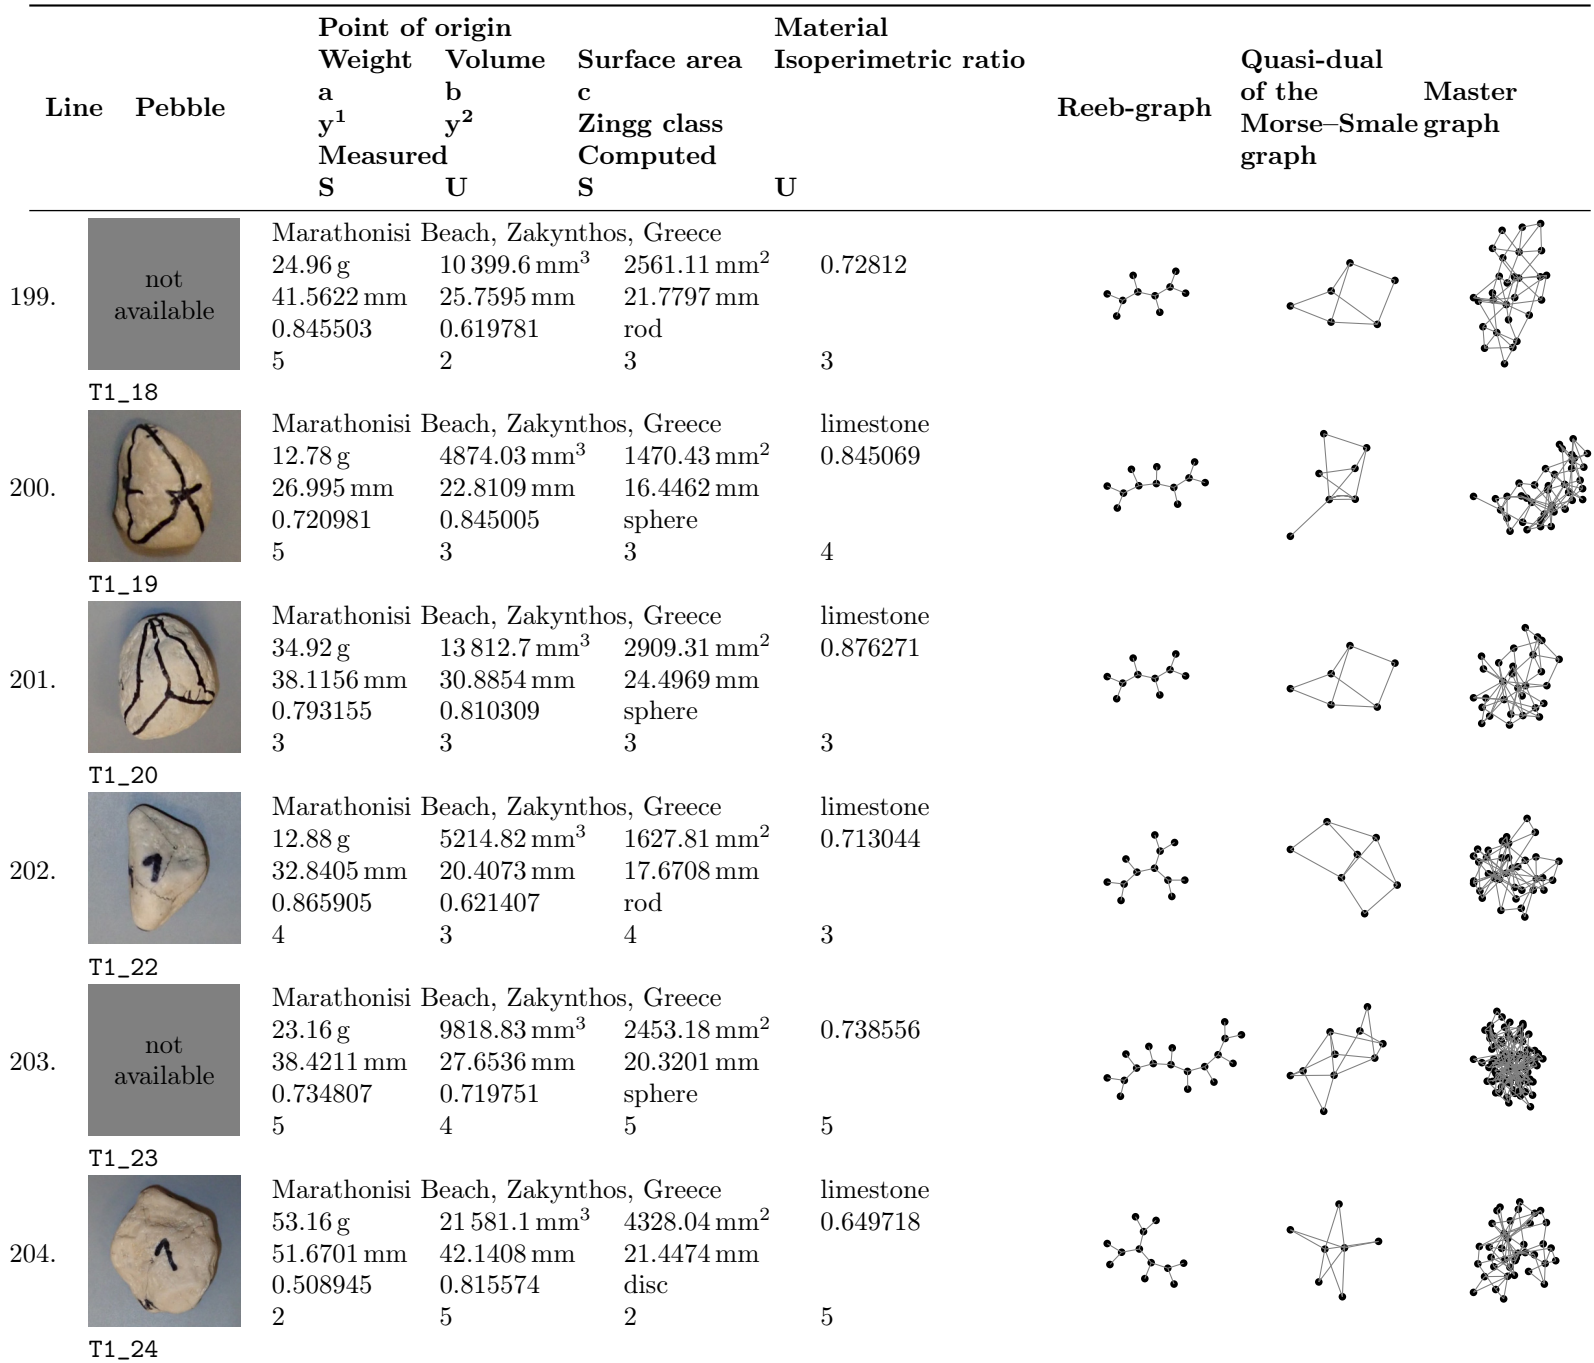   | 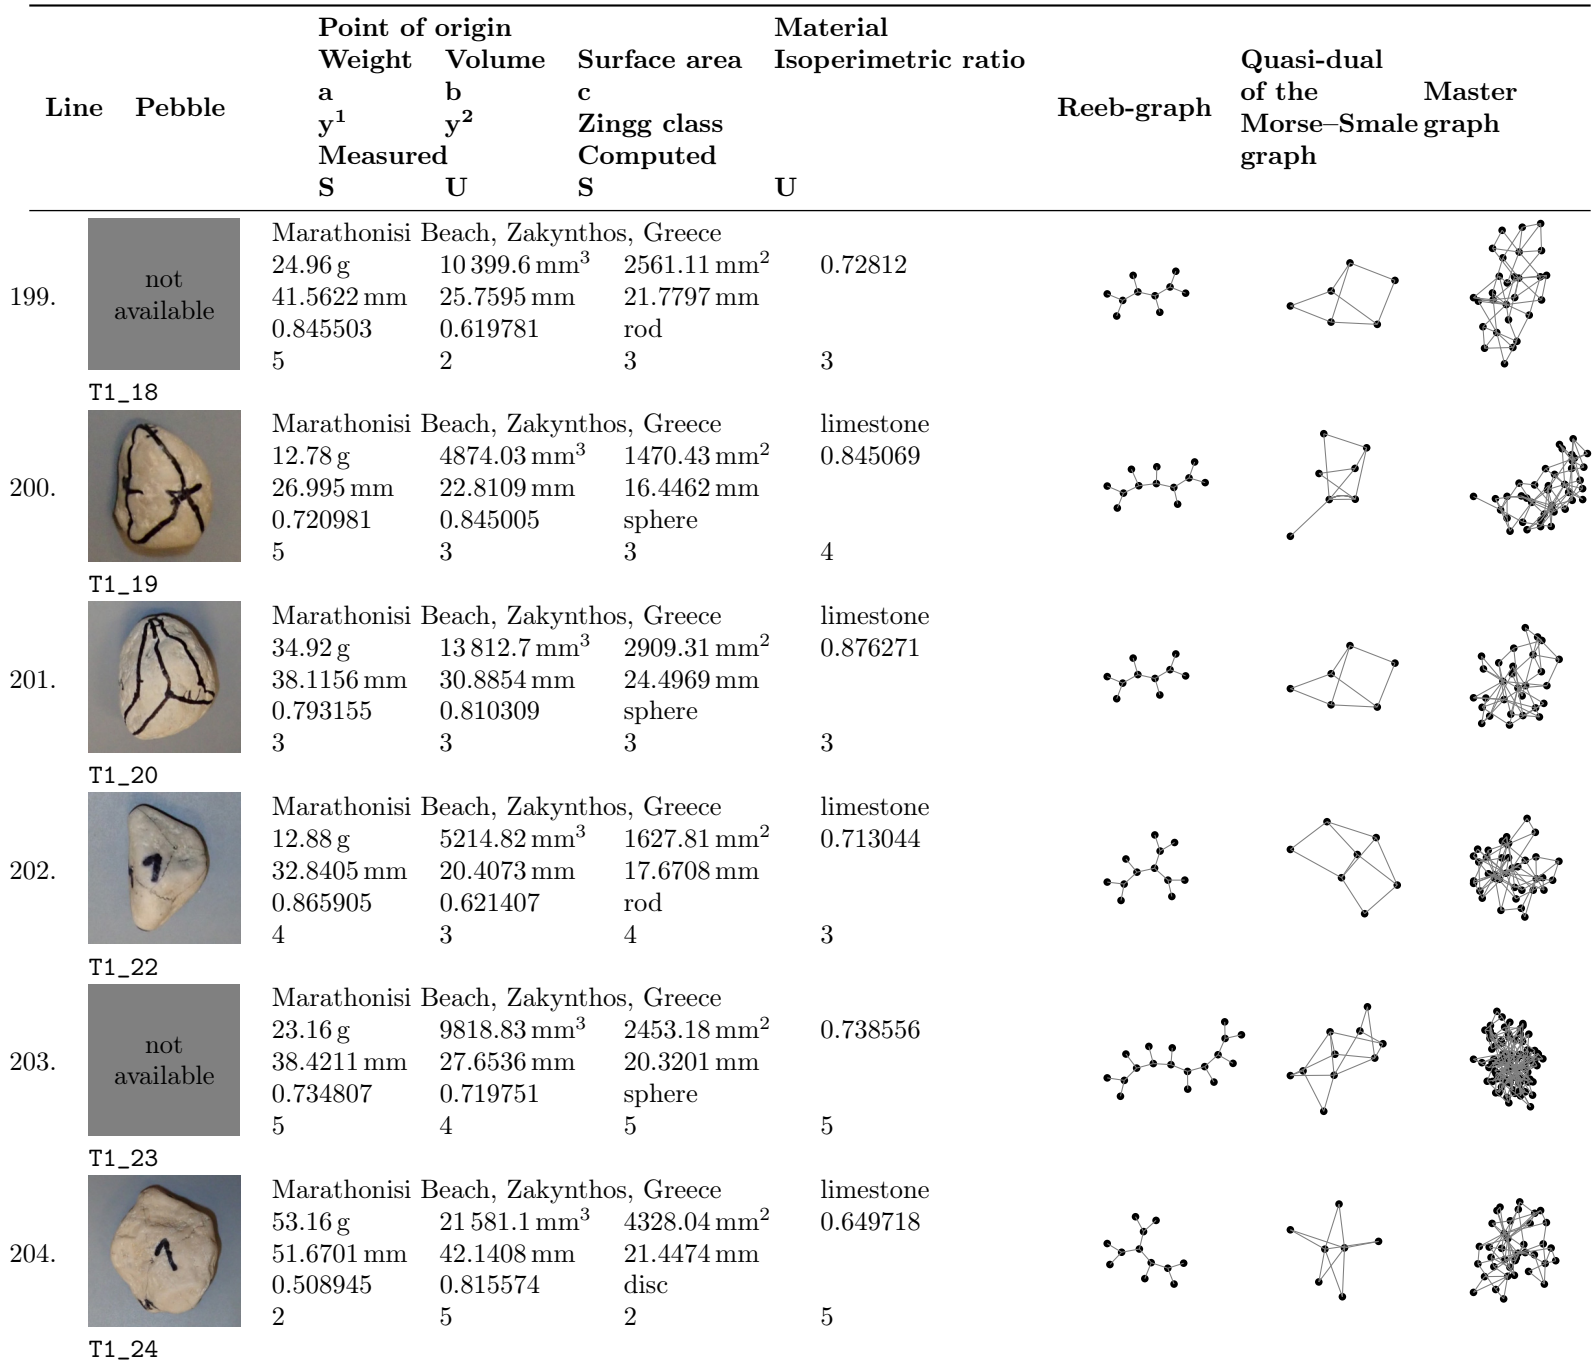   | 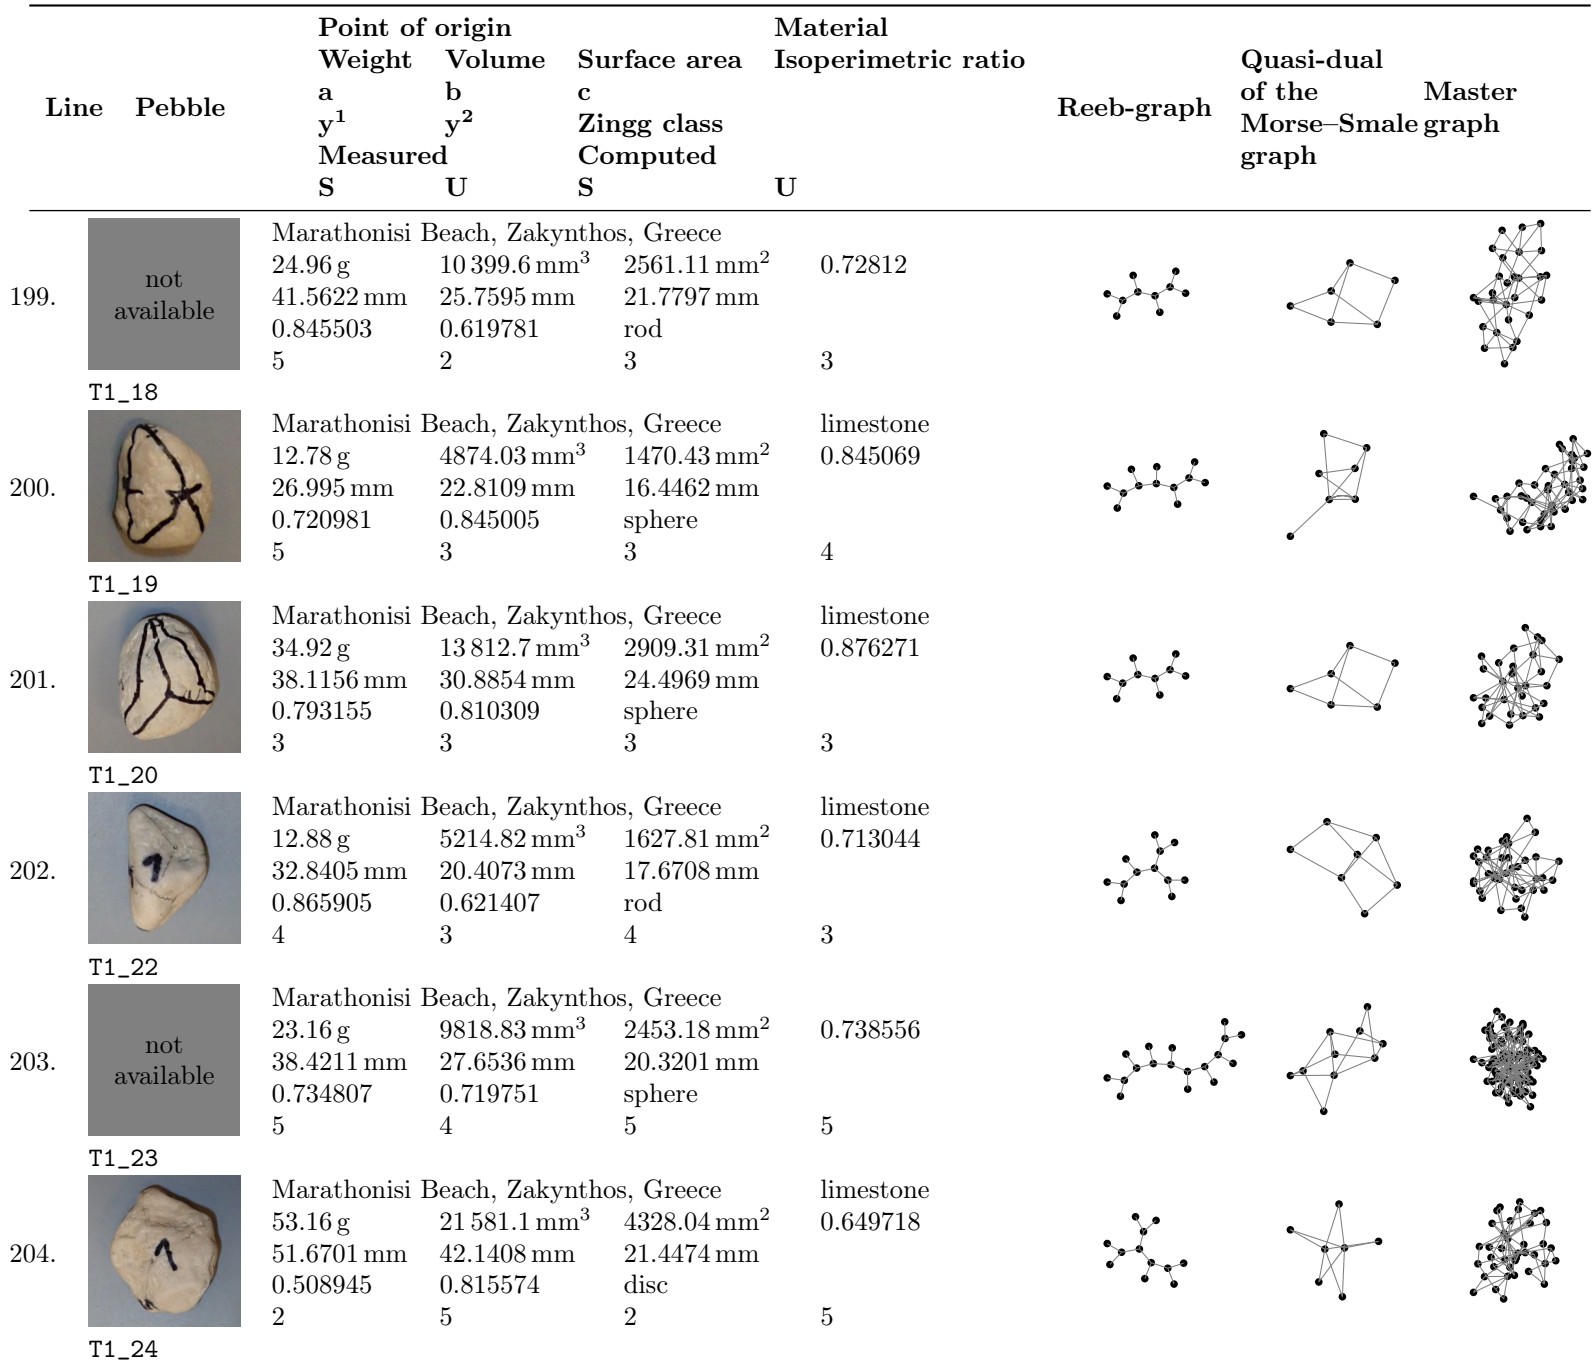   |
|      | T1_19                                                                               |                                                                                |                                                                    |                                                      |                                      |                                                                                       |                                                                                       |                                                                                       |
| 201. | 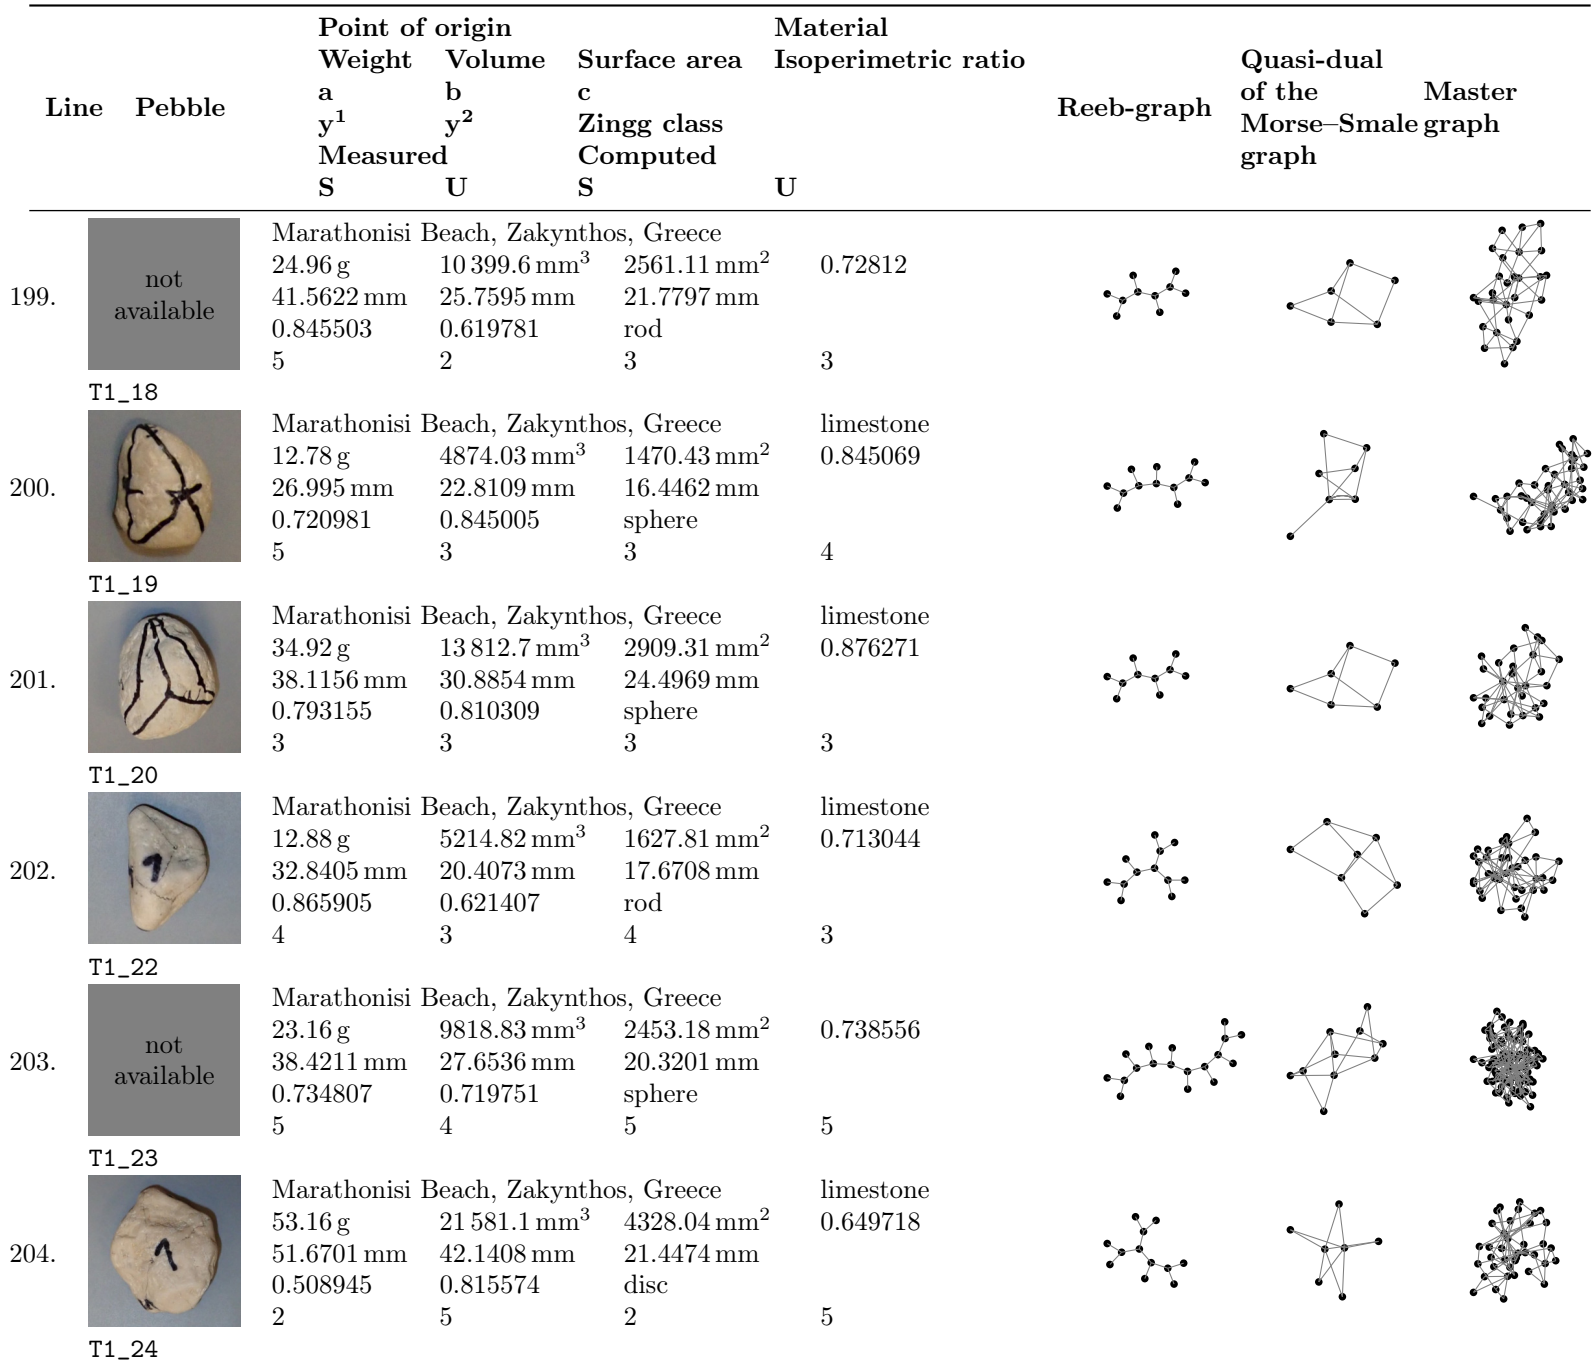   | Marathonisi Beach, Zakynthos, Greece<br>34.92 g<br>38.1156 mm<br>0.793155<br>3 | 34.92 g<br>13 812.7 mm <sup>3</sup><br>30.8854 mm<br>0.810309<br>3 | 2909.31 mm <sup>2</sup><br>24.4969 mm<br>sphere<br>3 | limestone<br>0.876271<br><br>3       | 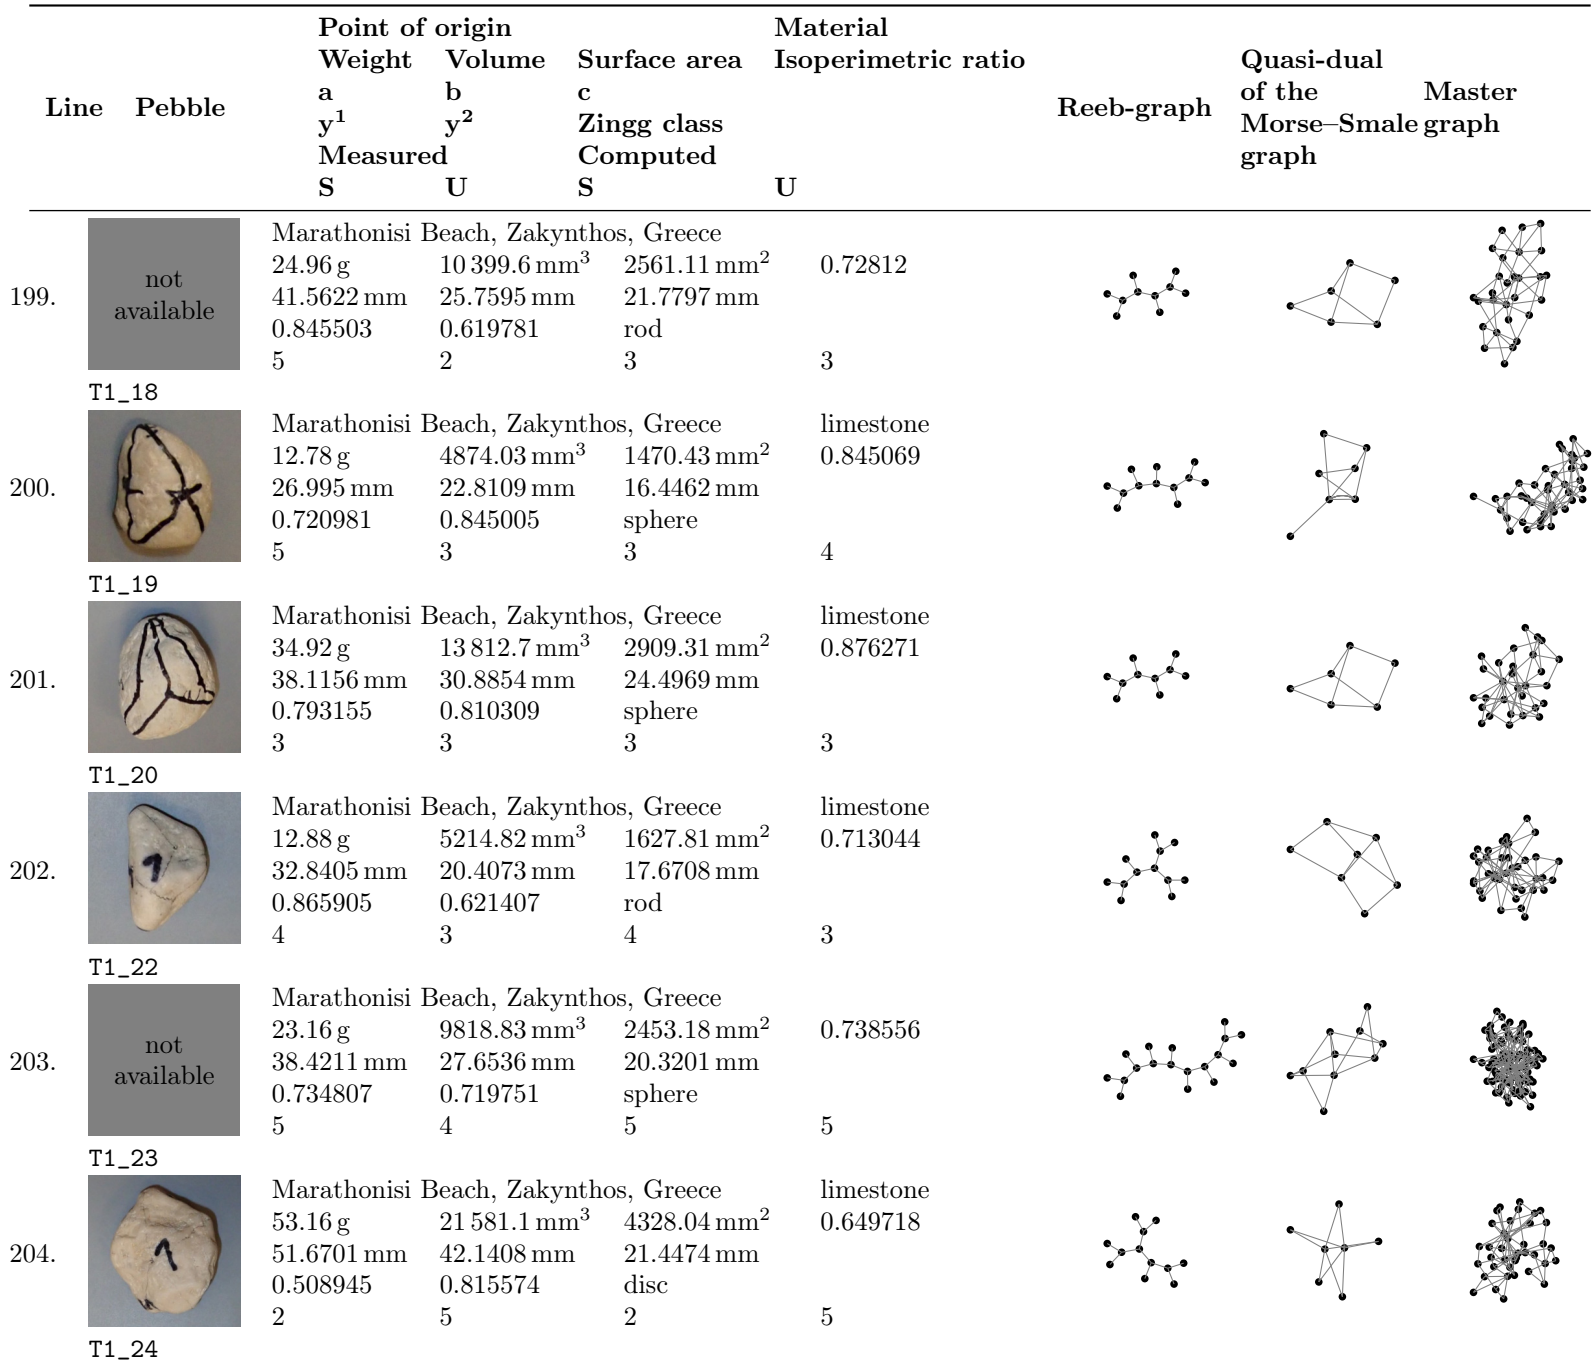   | 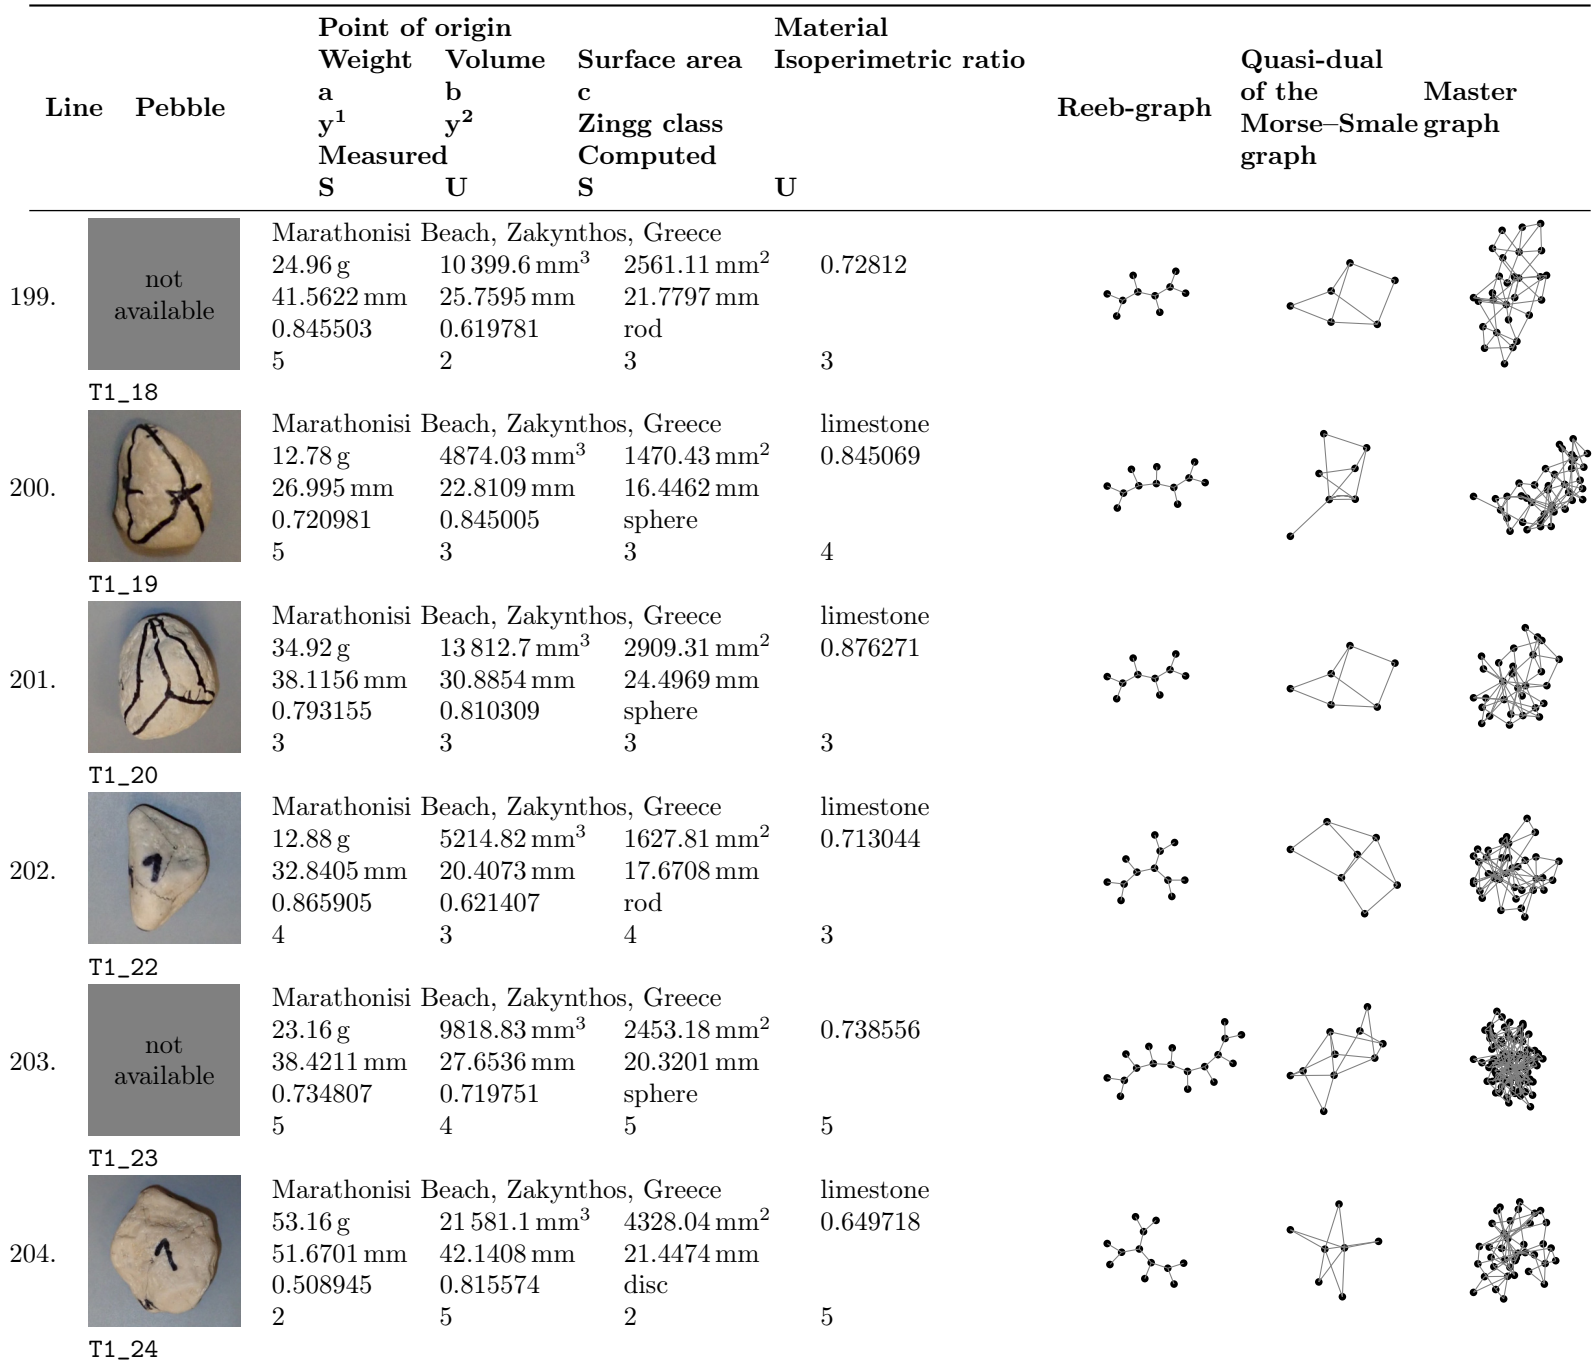   | 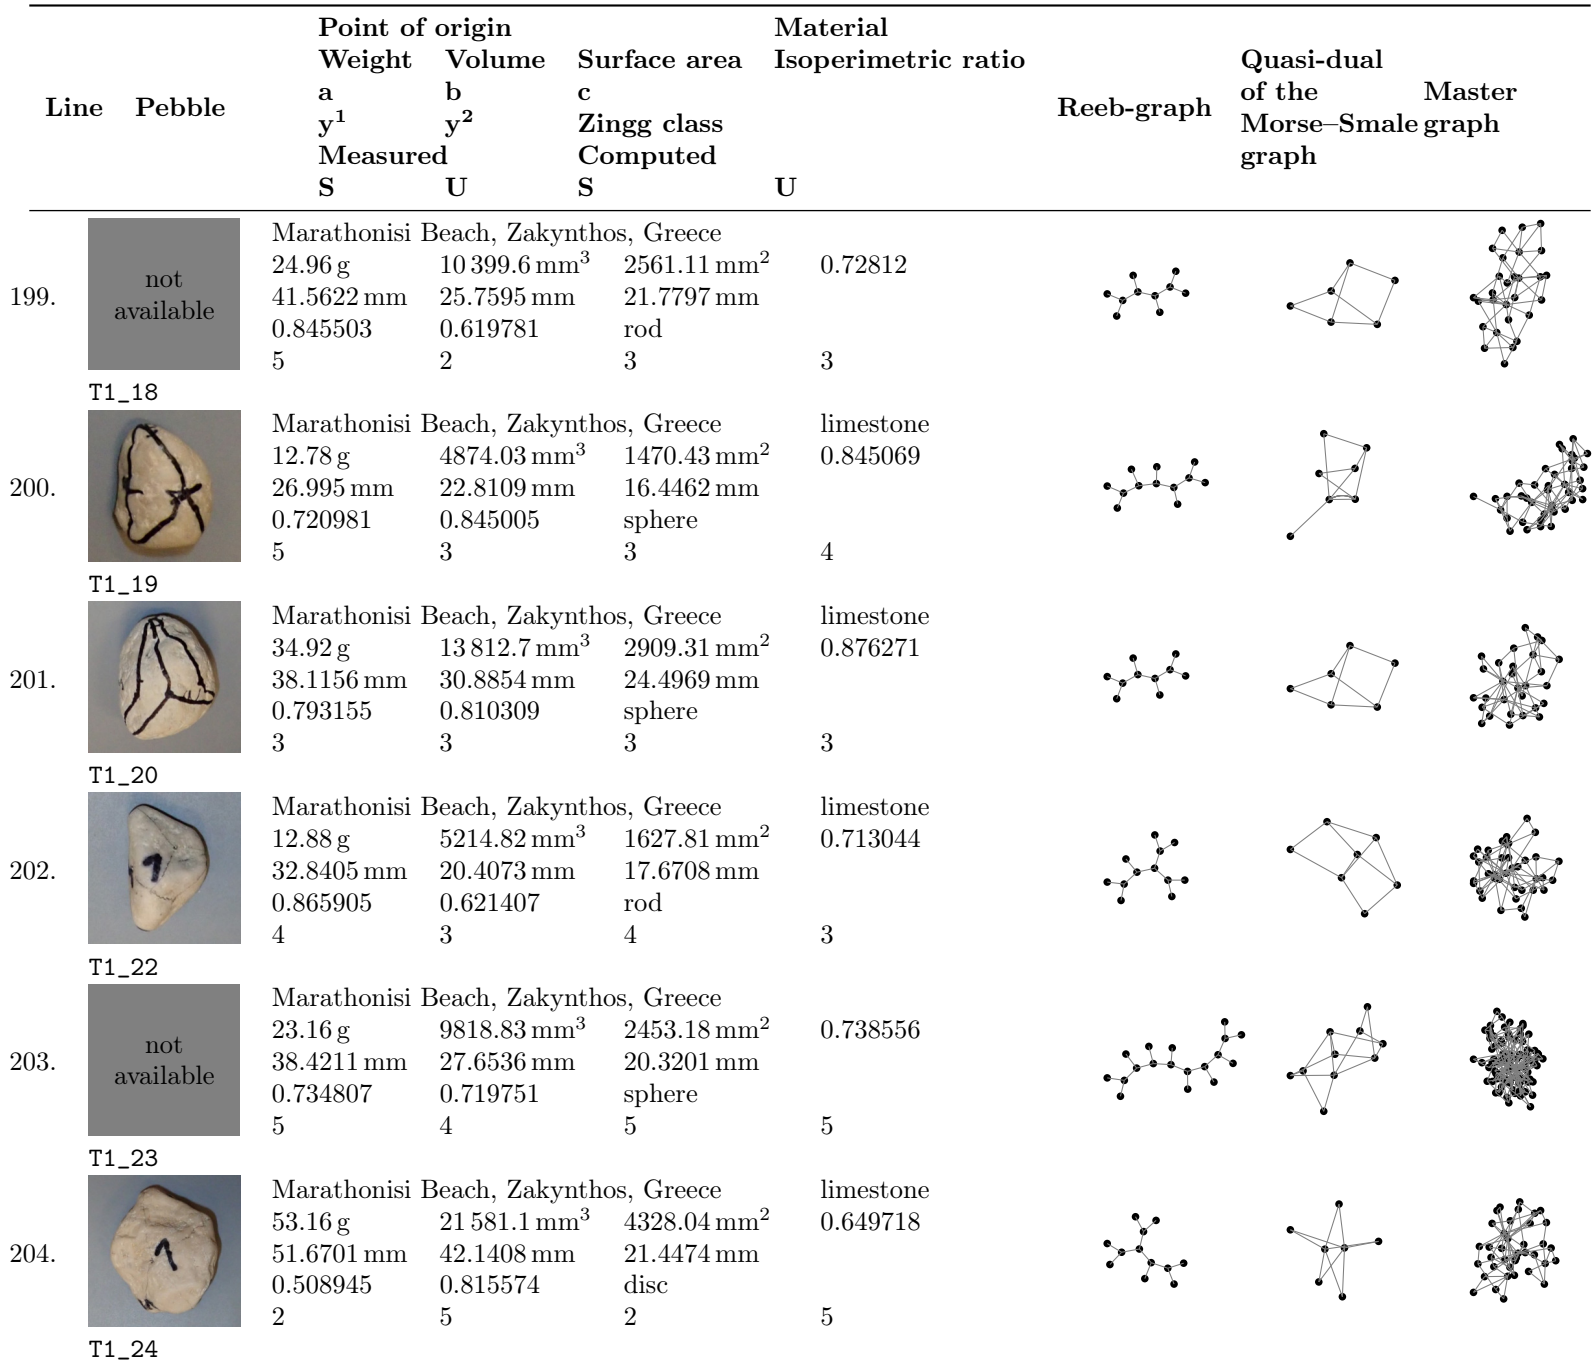   |
|      | T1_20                                                                               |                                                                                |                                                                    |                                                      |                                      |                                                                                       |                                                                                       |                                                                                       |
| 202. | 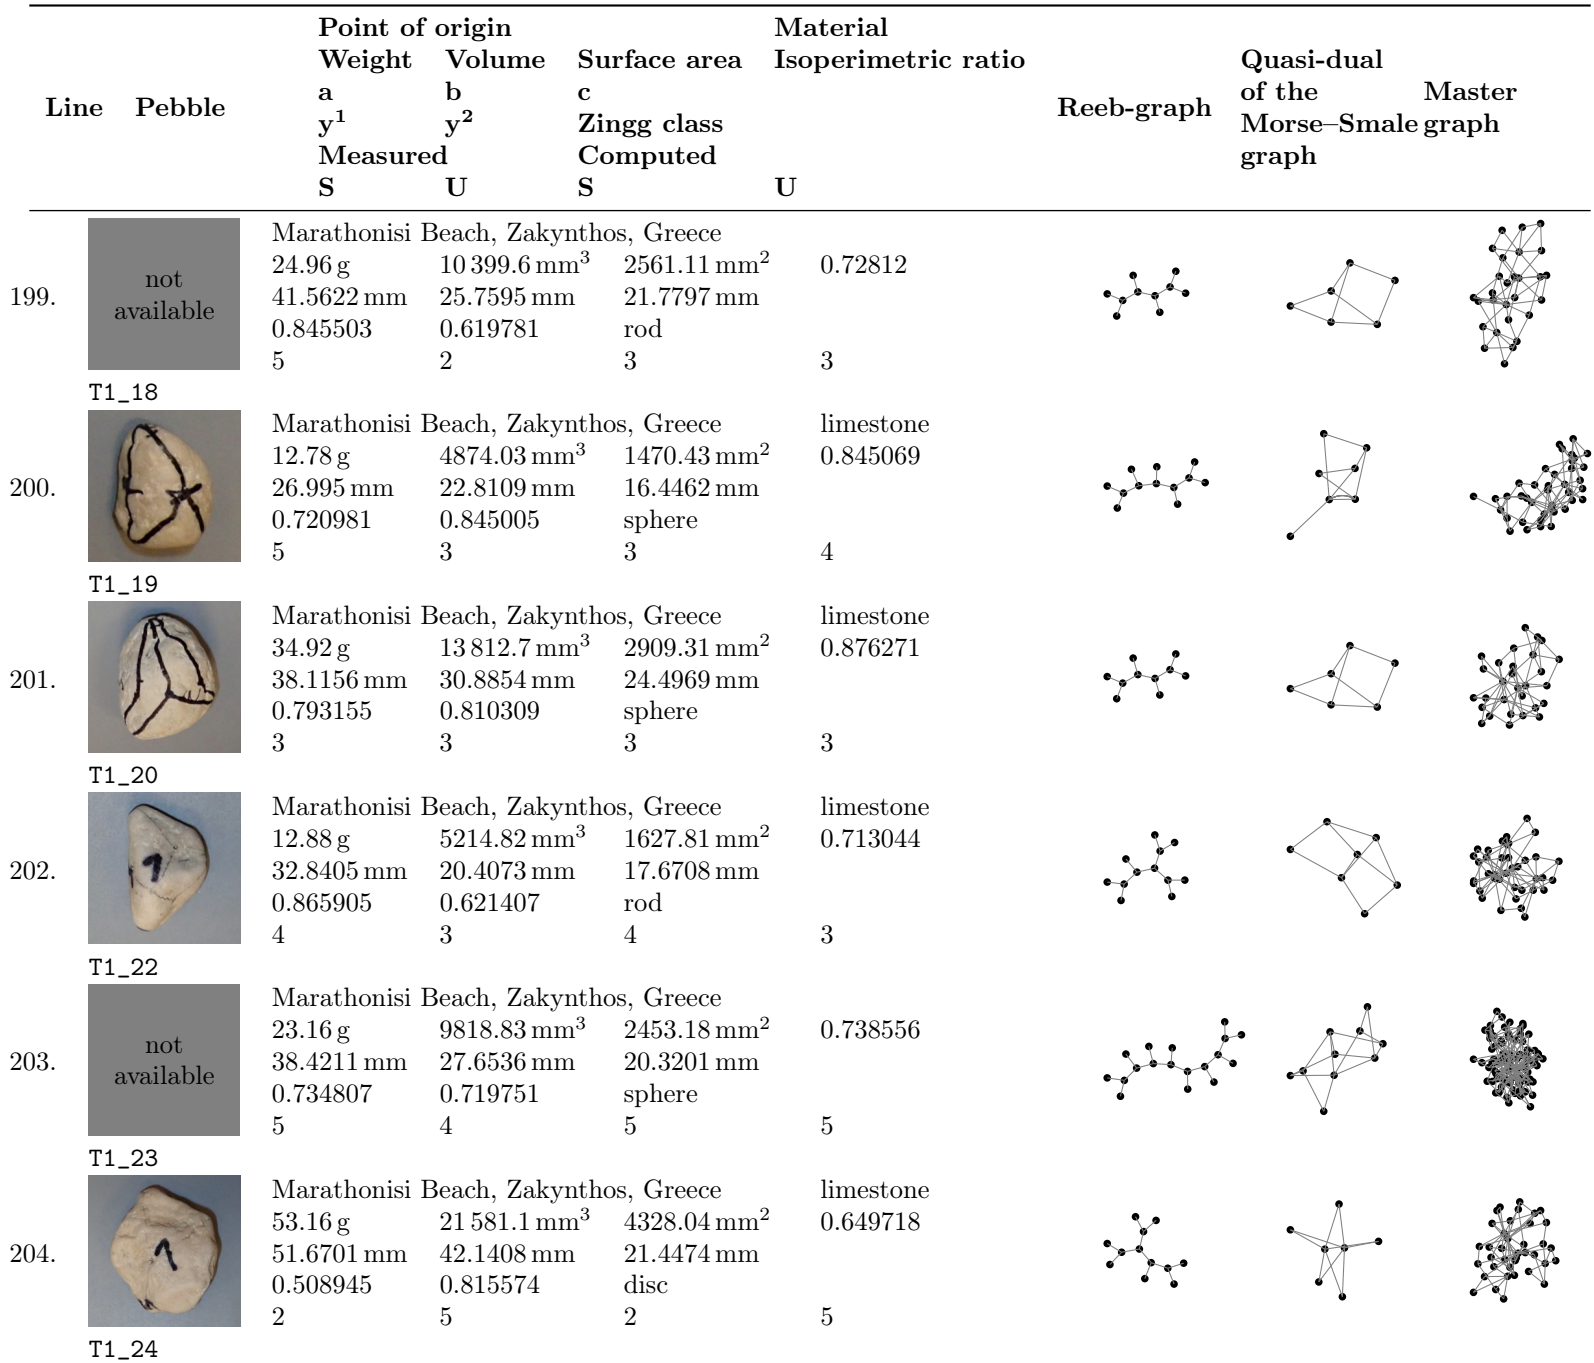  | Marathonisi Beach, Zakynthos, Greece<br>12.88 g<br>32.8405 mm<br>0.865905<br>4 | 12.88 g<br>5214.82 mm <sup>3</sup><br>20.4073 mm<br>0.621407<br>3  | 1627.81 mm <sup>2</sup><br>17.6708 mm<br>rod<br>4    | limestone<br>0.713044<br><br>3       | 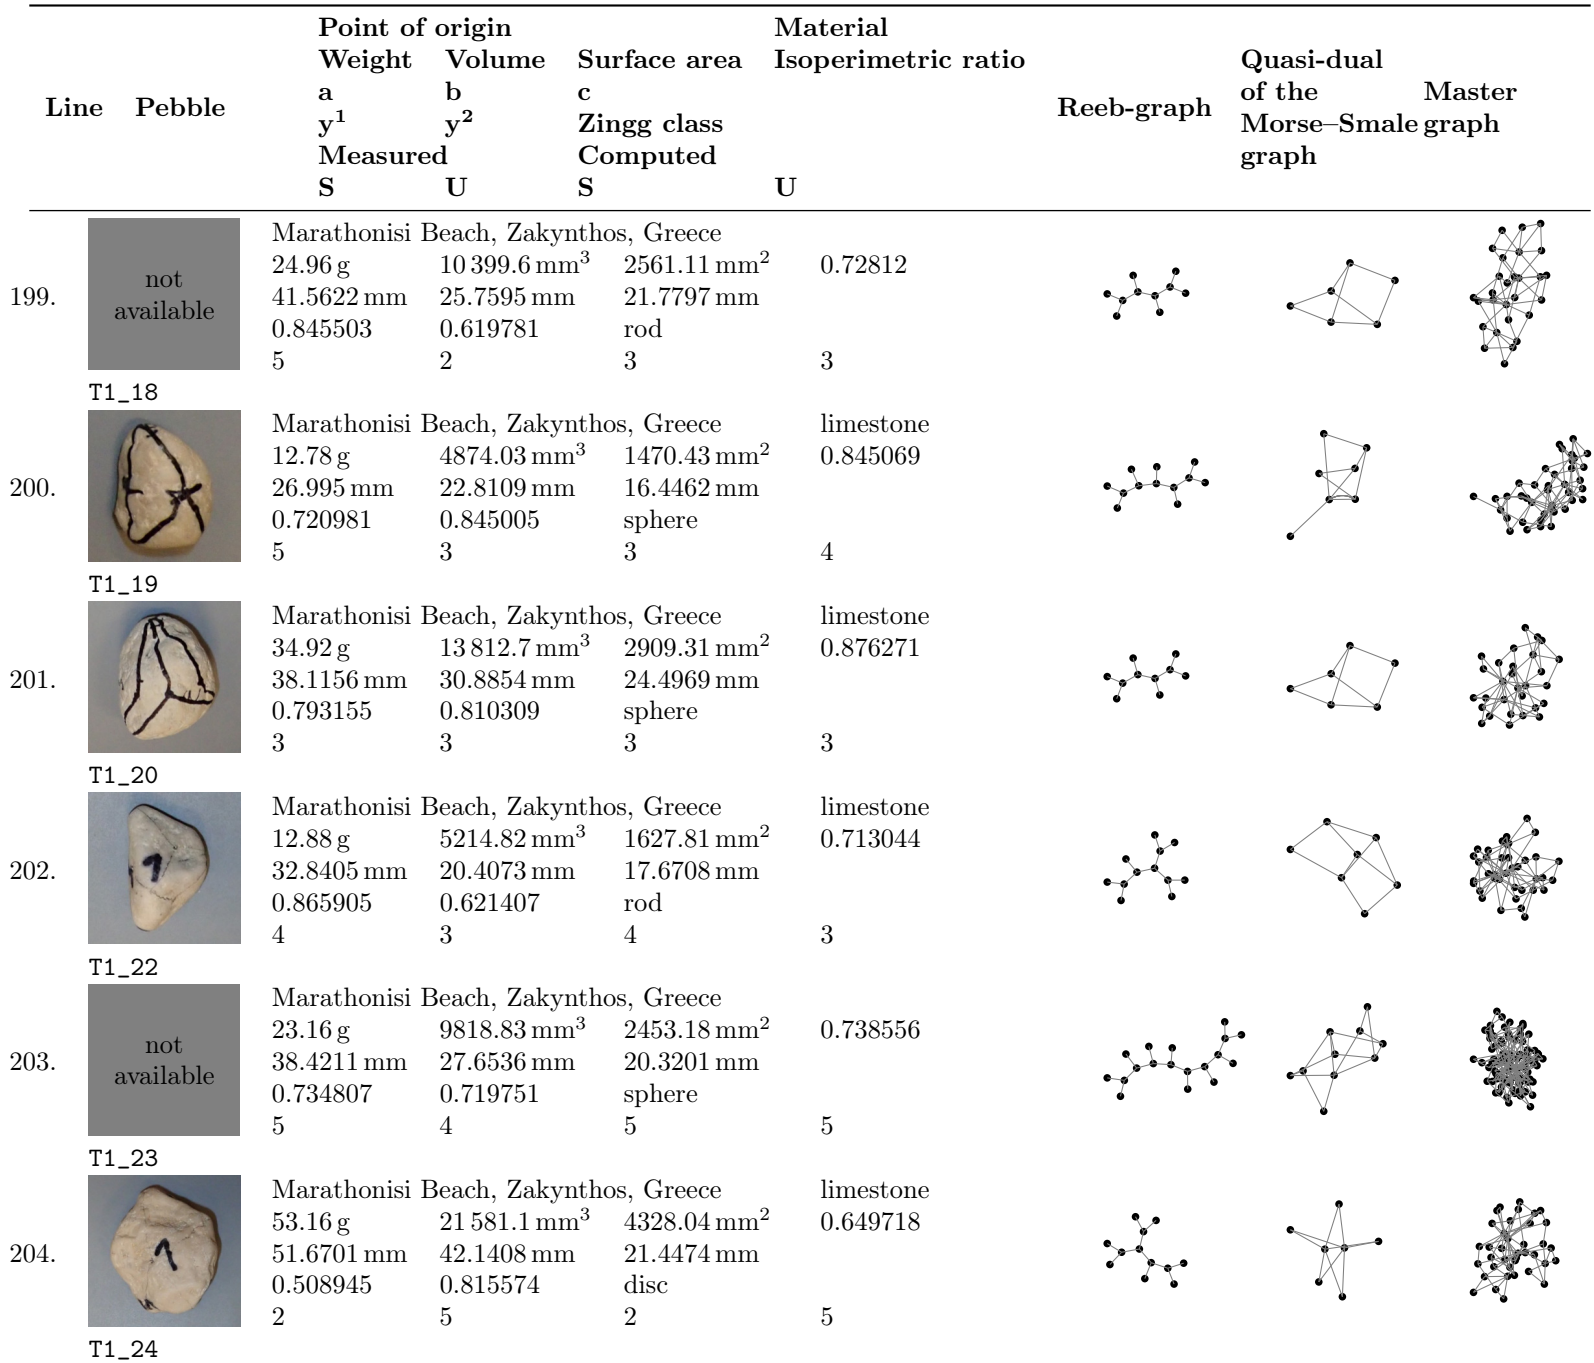  | 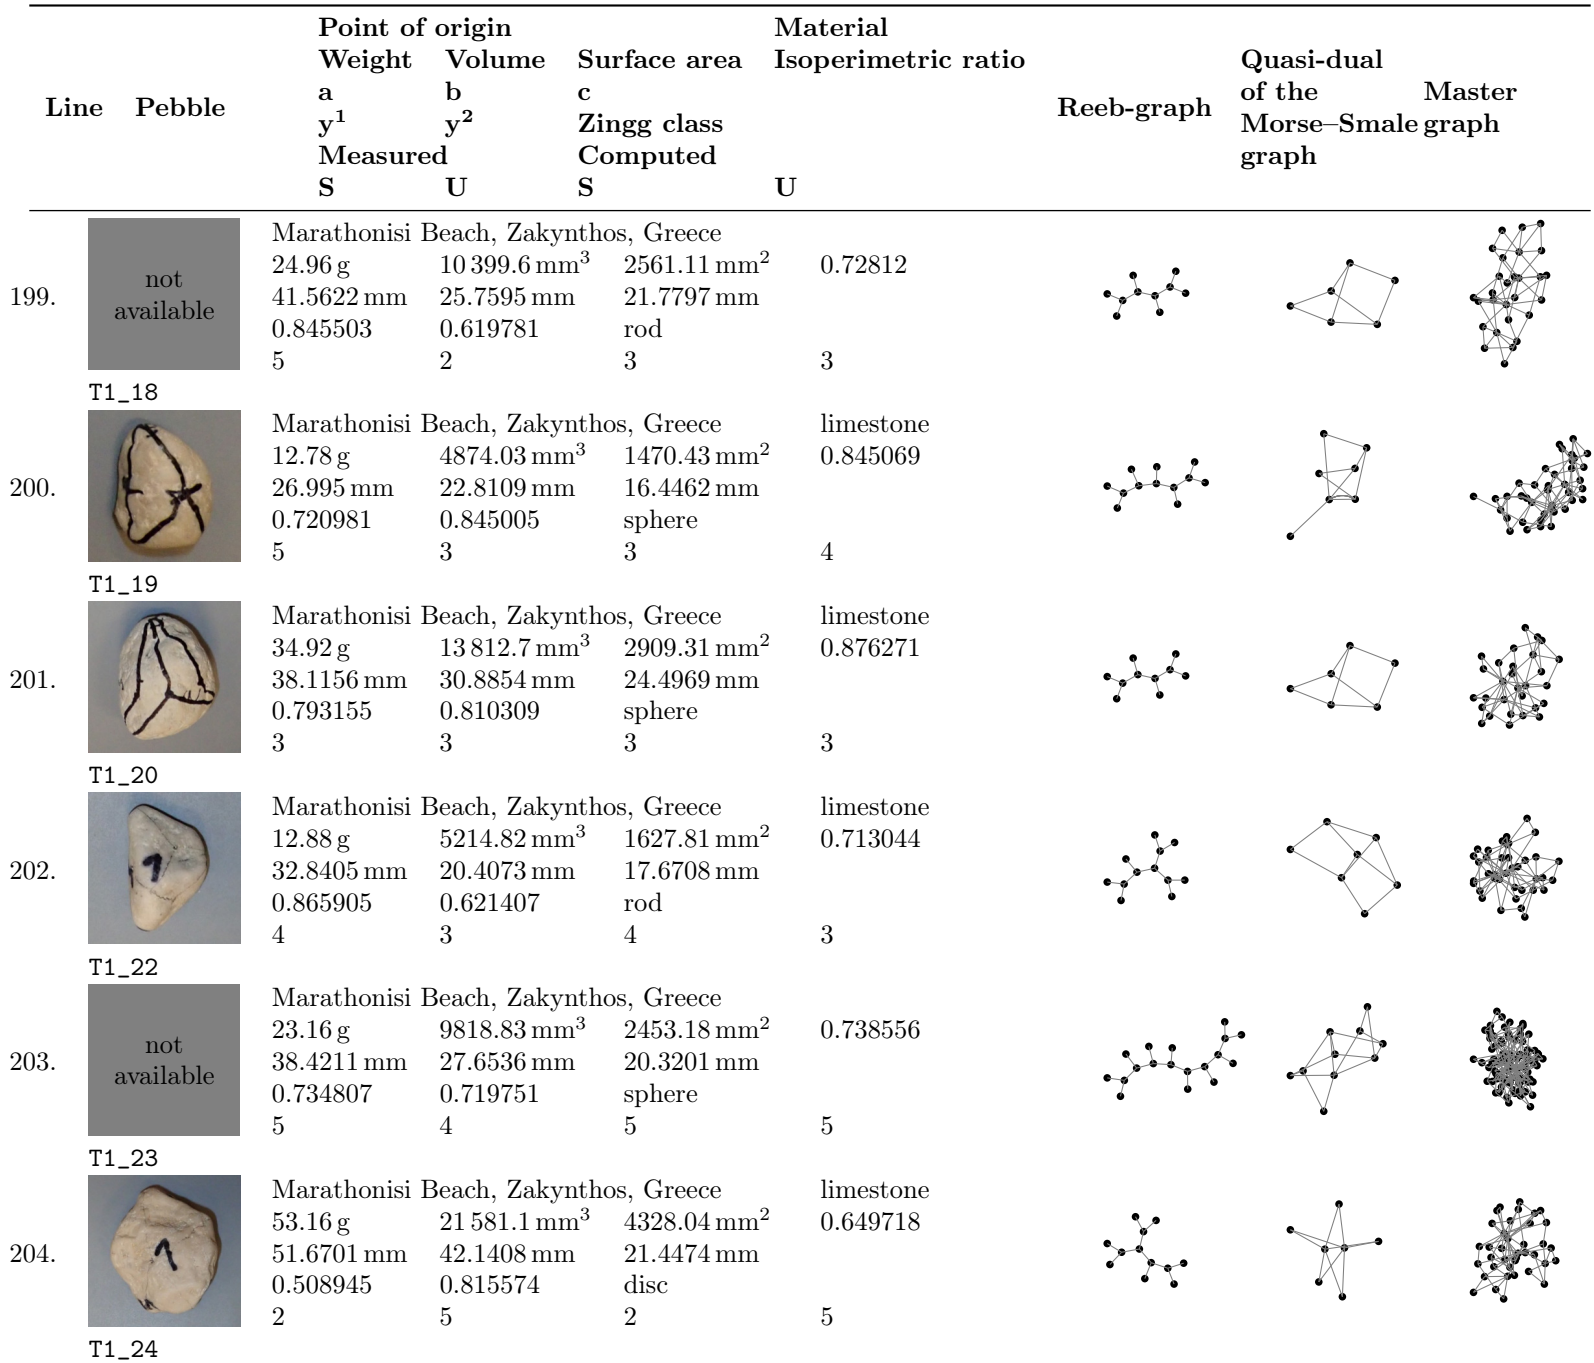  | 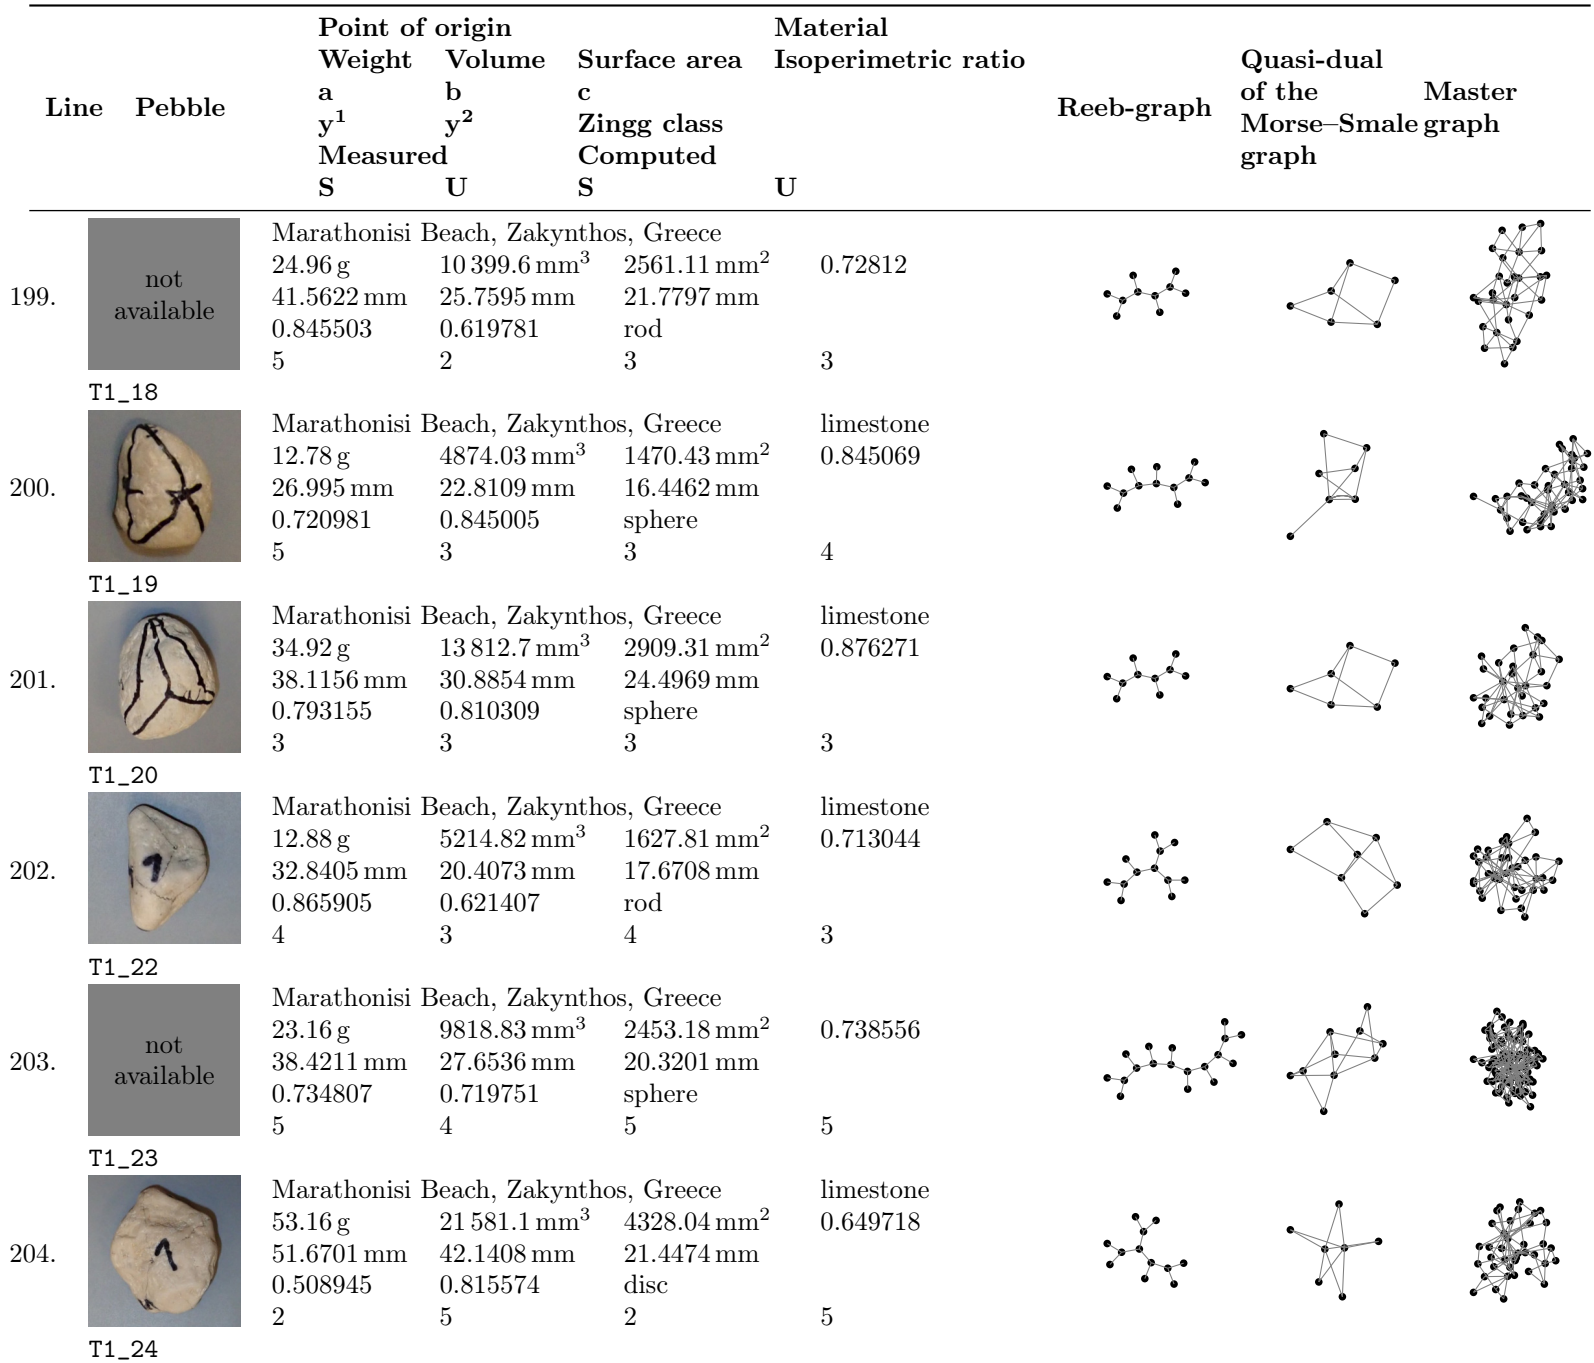  |
|      | T1_22                                                                               |                                                                                |                                                                    |                                                      |                                      |                                                                                       |                                                                                       |                                                                                       |
| 203. | 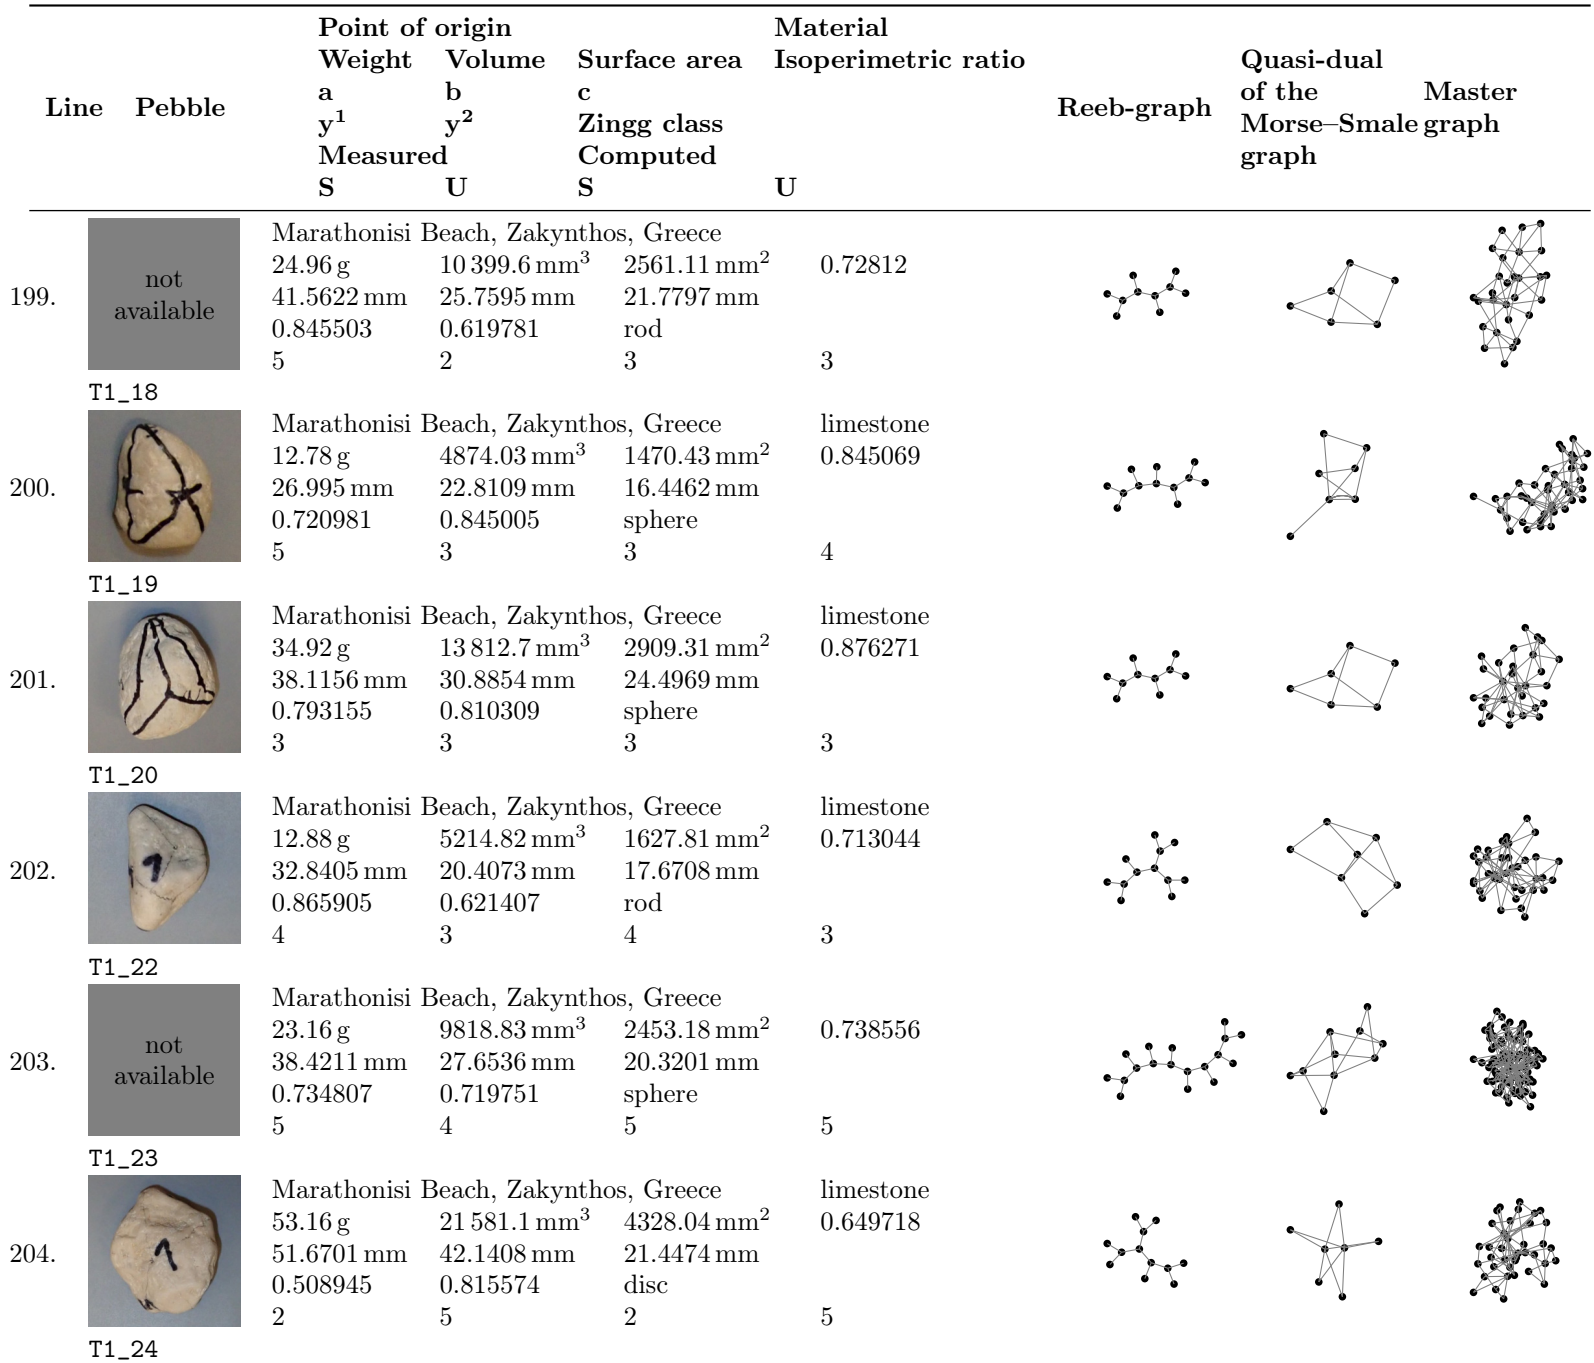 | Marathonisi Beach, Zakynthos, Greece<br>23.16 g<br>38.4211 mm<br>0.734807<br>5 | 23.16 g<br>9818.83 mm <sup>3</sup><br>27.6536 mm<br>0.719751<br>4  | 2453.18 mm <sup>2</sup><br>20.3201 mm<br>sphere<br>5 | 0.738556<br><br><br>5                | 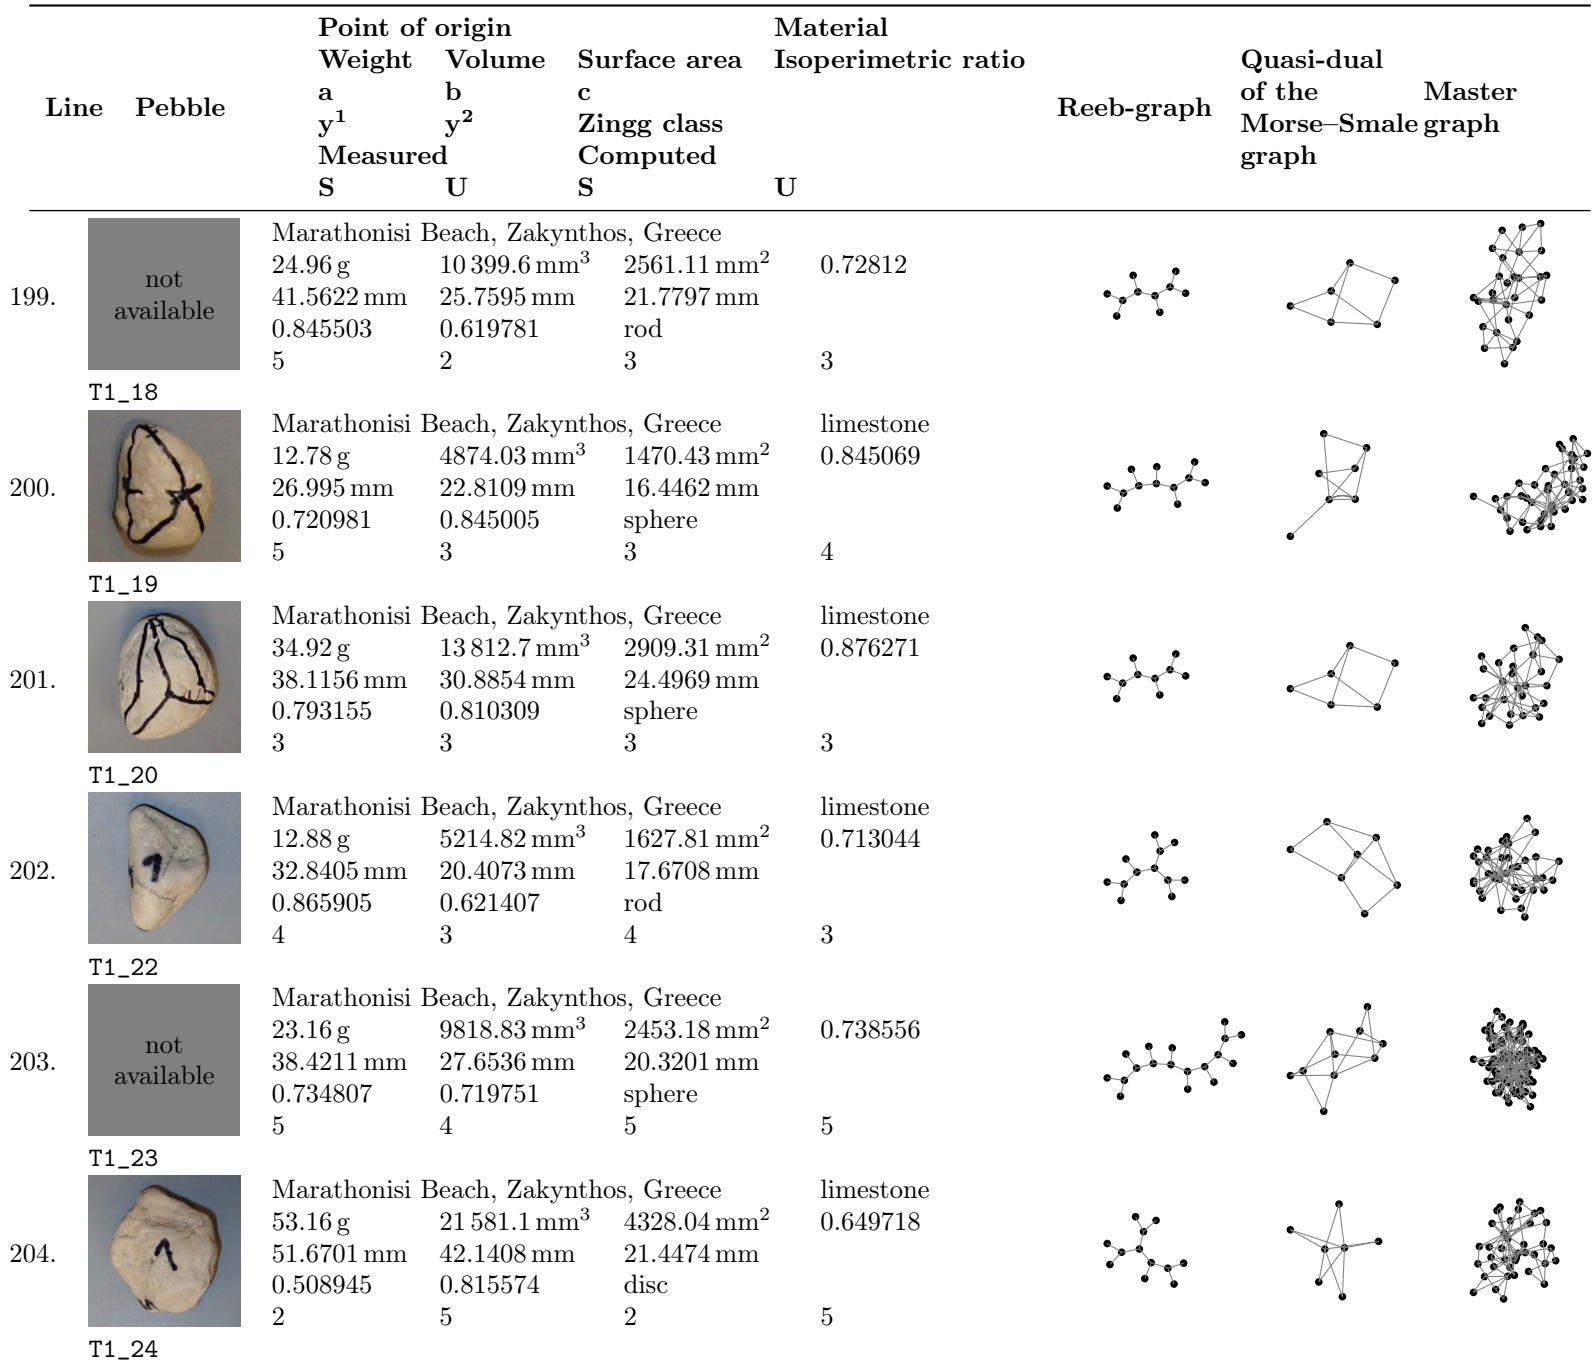 | 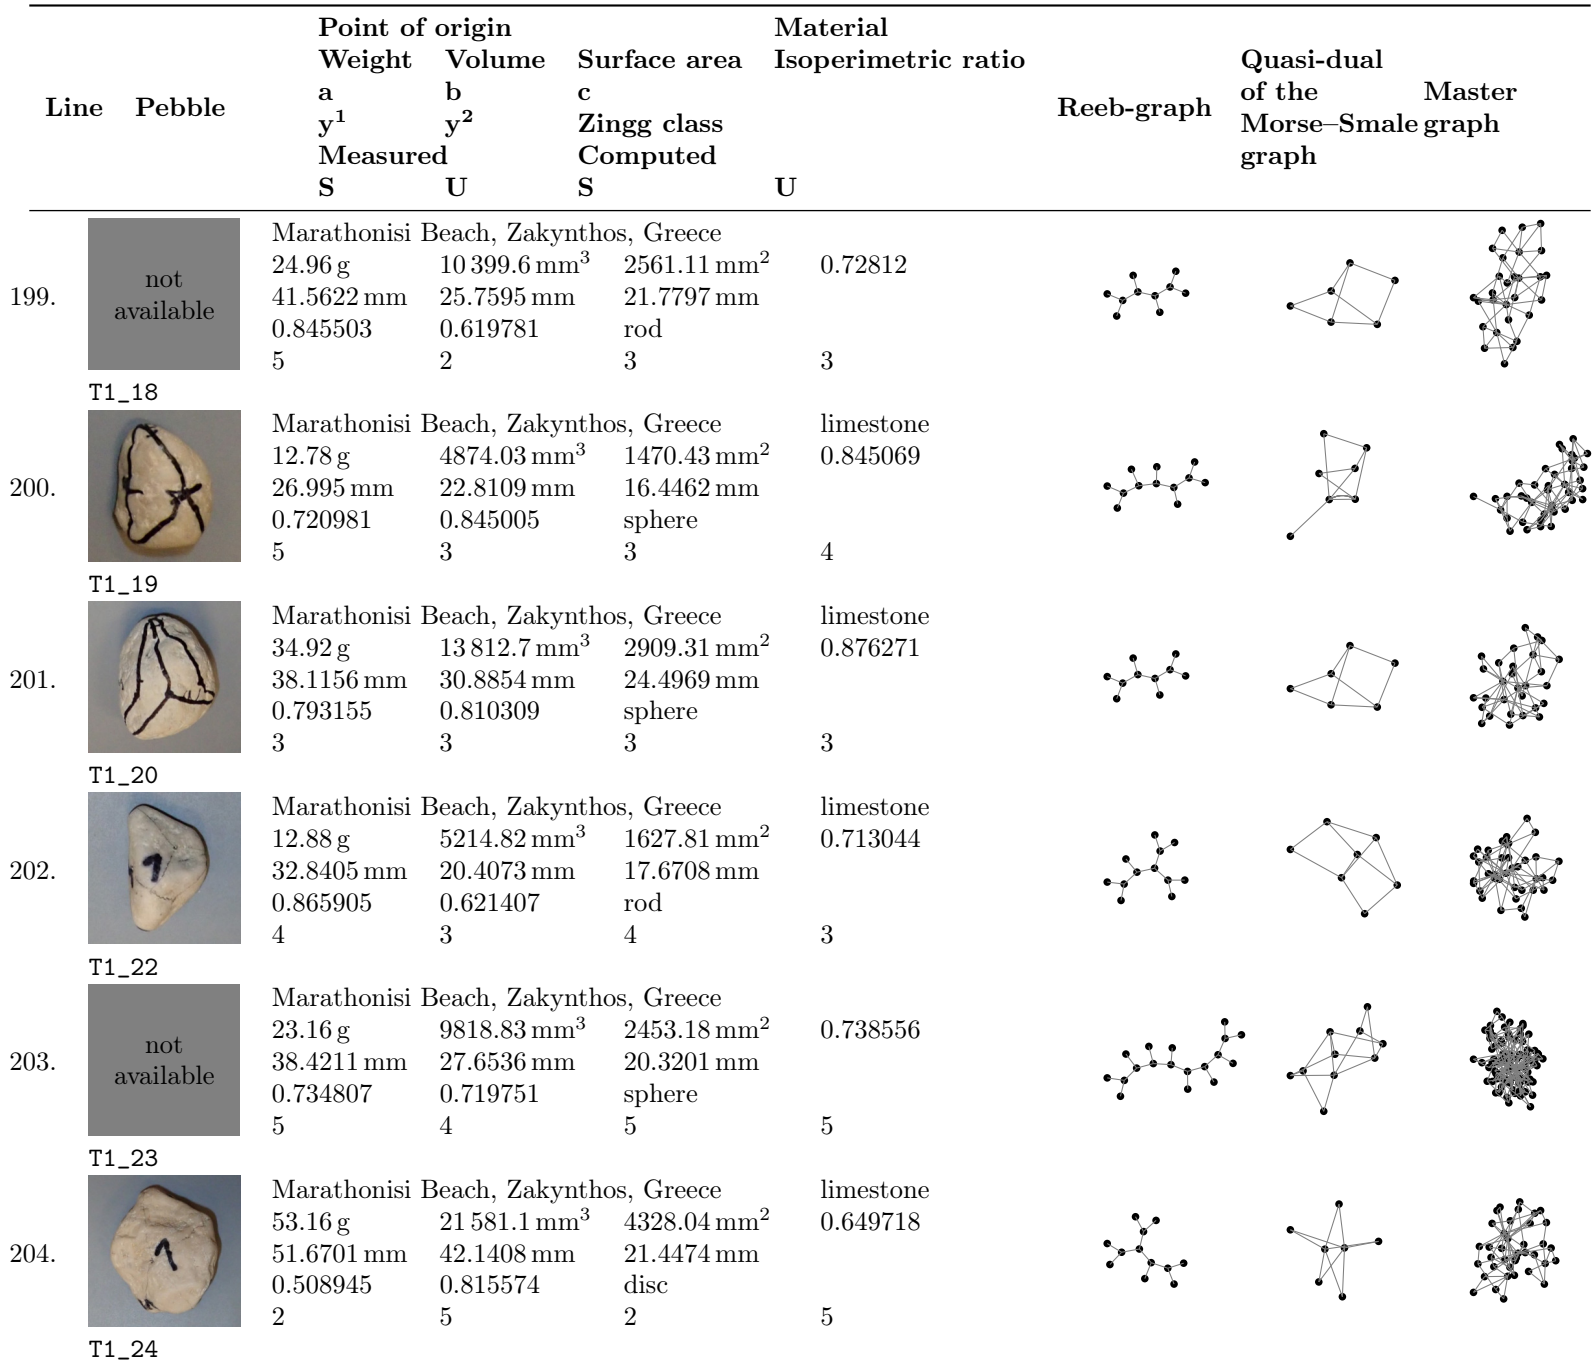 | 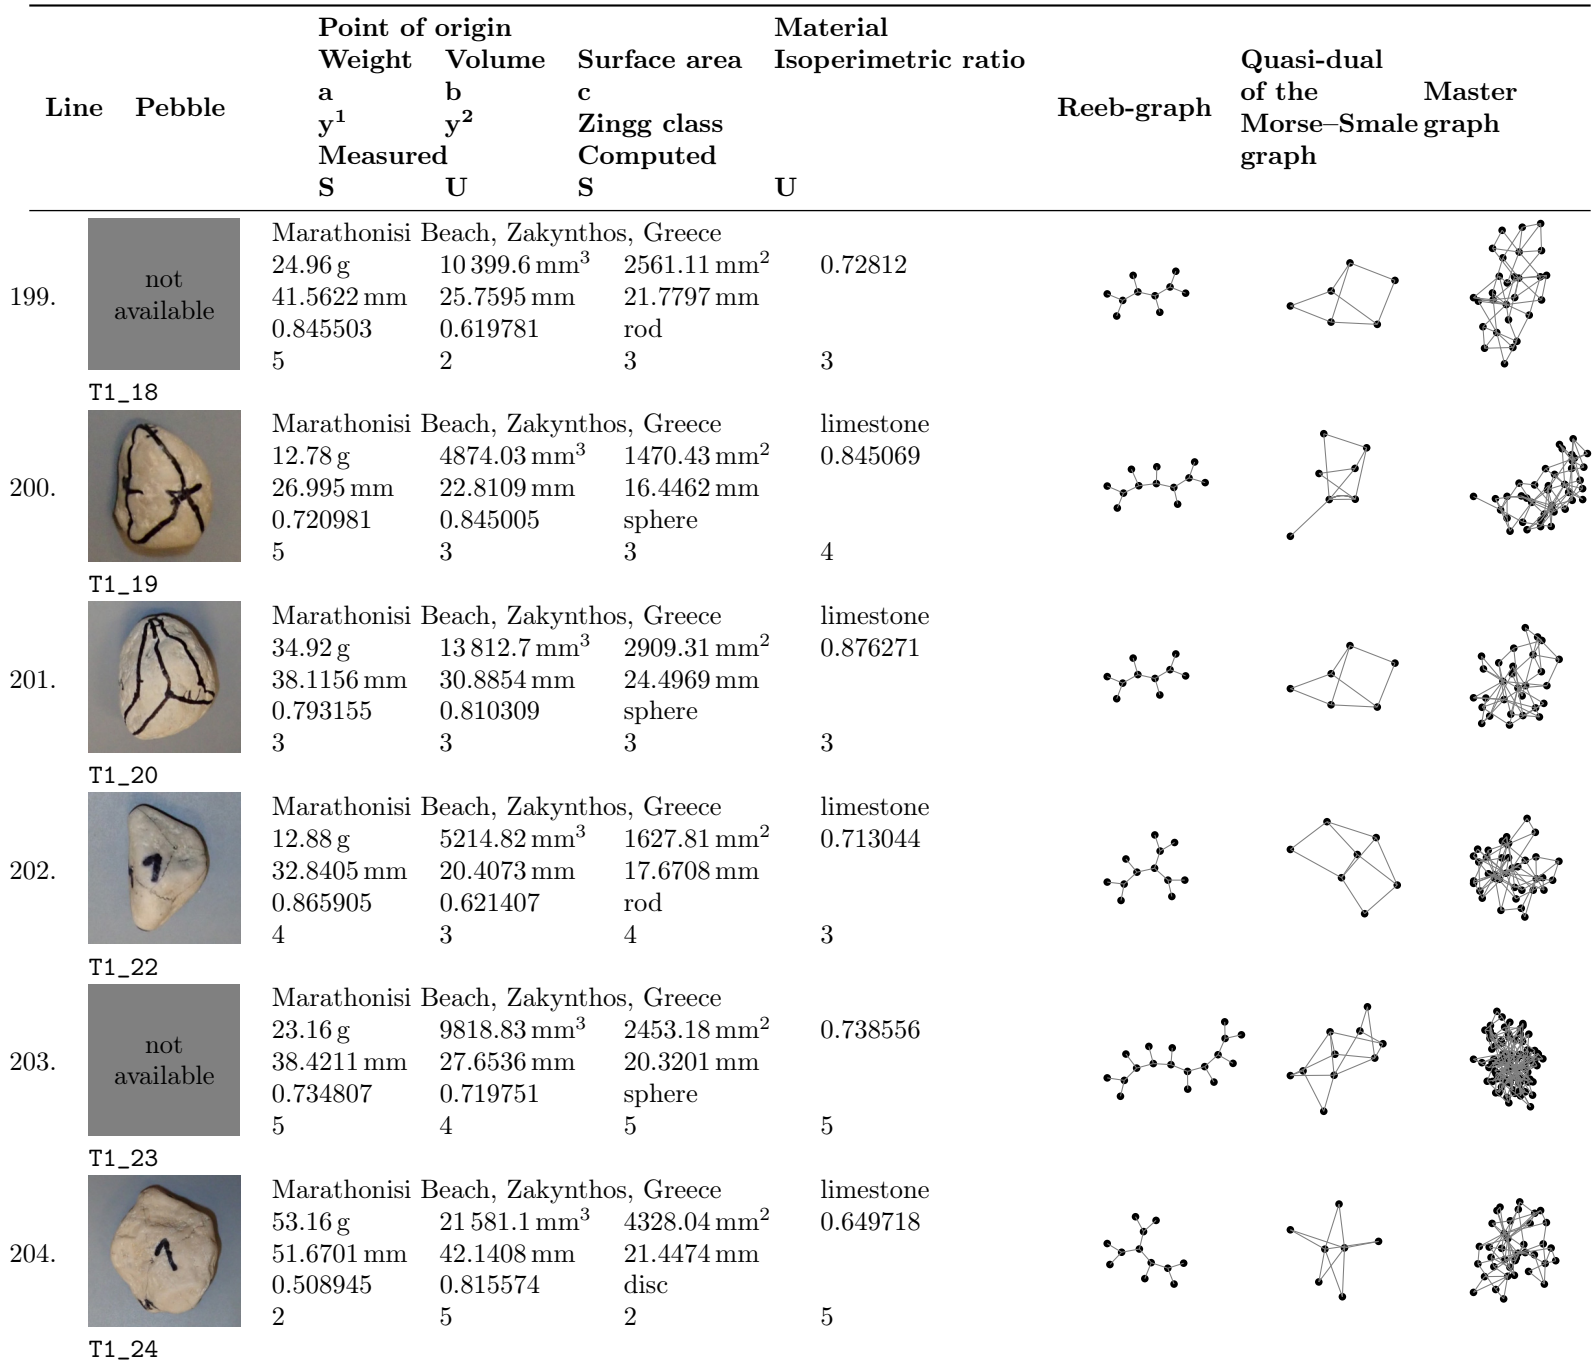 |
|      | T1_23                                                                               |                                                                                |                                                                    |                                                      |                                      |                                                                                       |                                                                                       |                                                                                       |
| 204. | 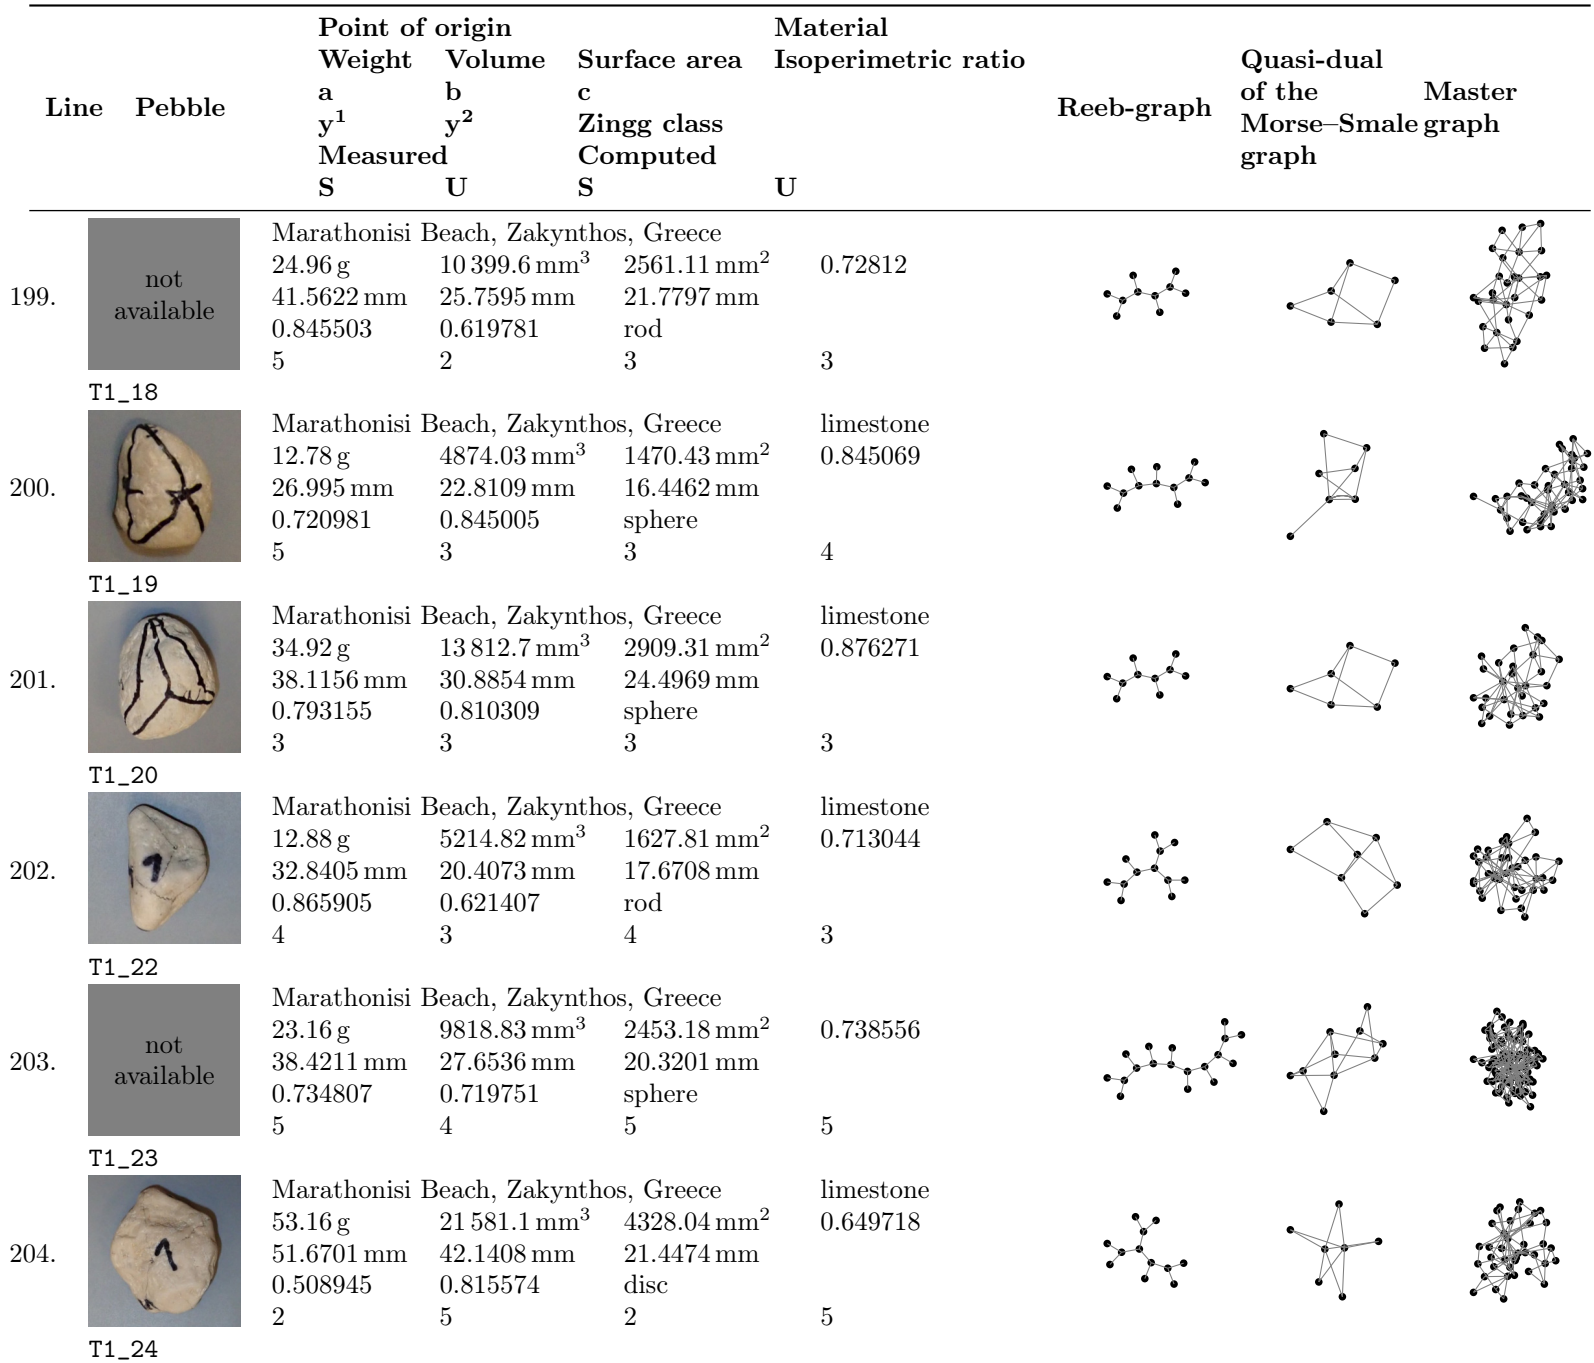 | Marathonisi Beach, Zakynthos, Greece<br>53.16 g<br>51.6701 mm<br>0.508945<br>2 | 53.16 g<br>21 581.1 mm <sup>3</sup><br>42.1408 mm<br>0.815574<br>5 | 4328.04 mm <sup>2</sup><br>21.4474 mm<br>disc<br>2   | limestone<br>0.649718<br><br>5       | 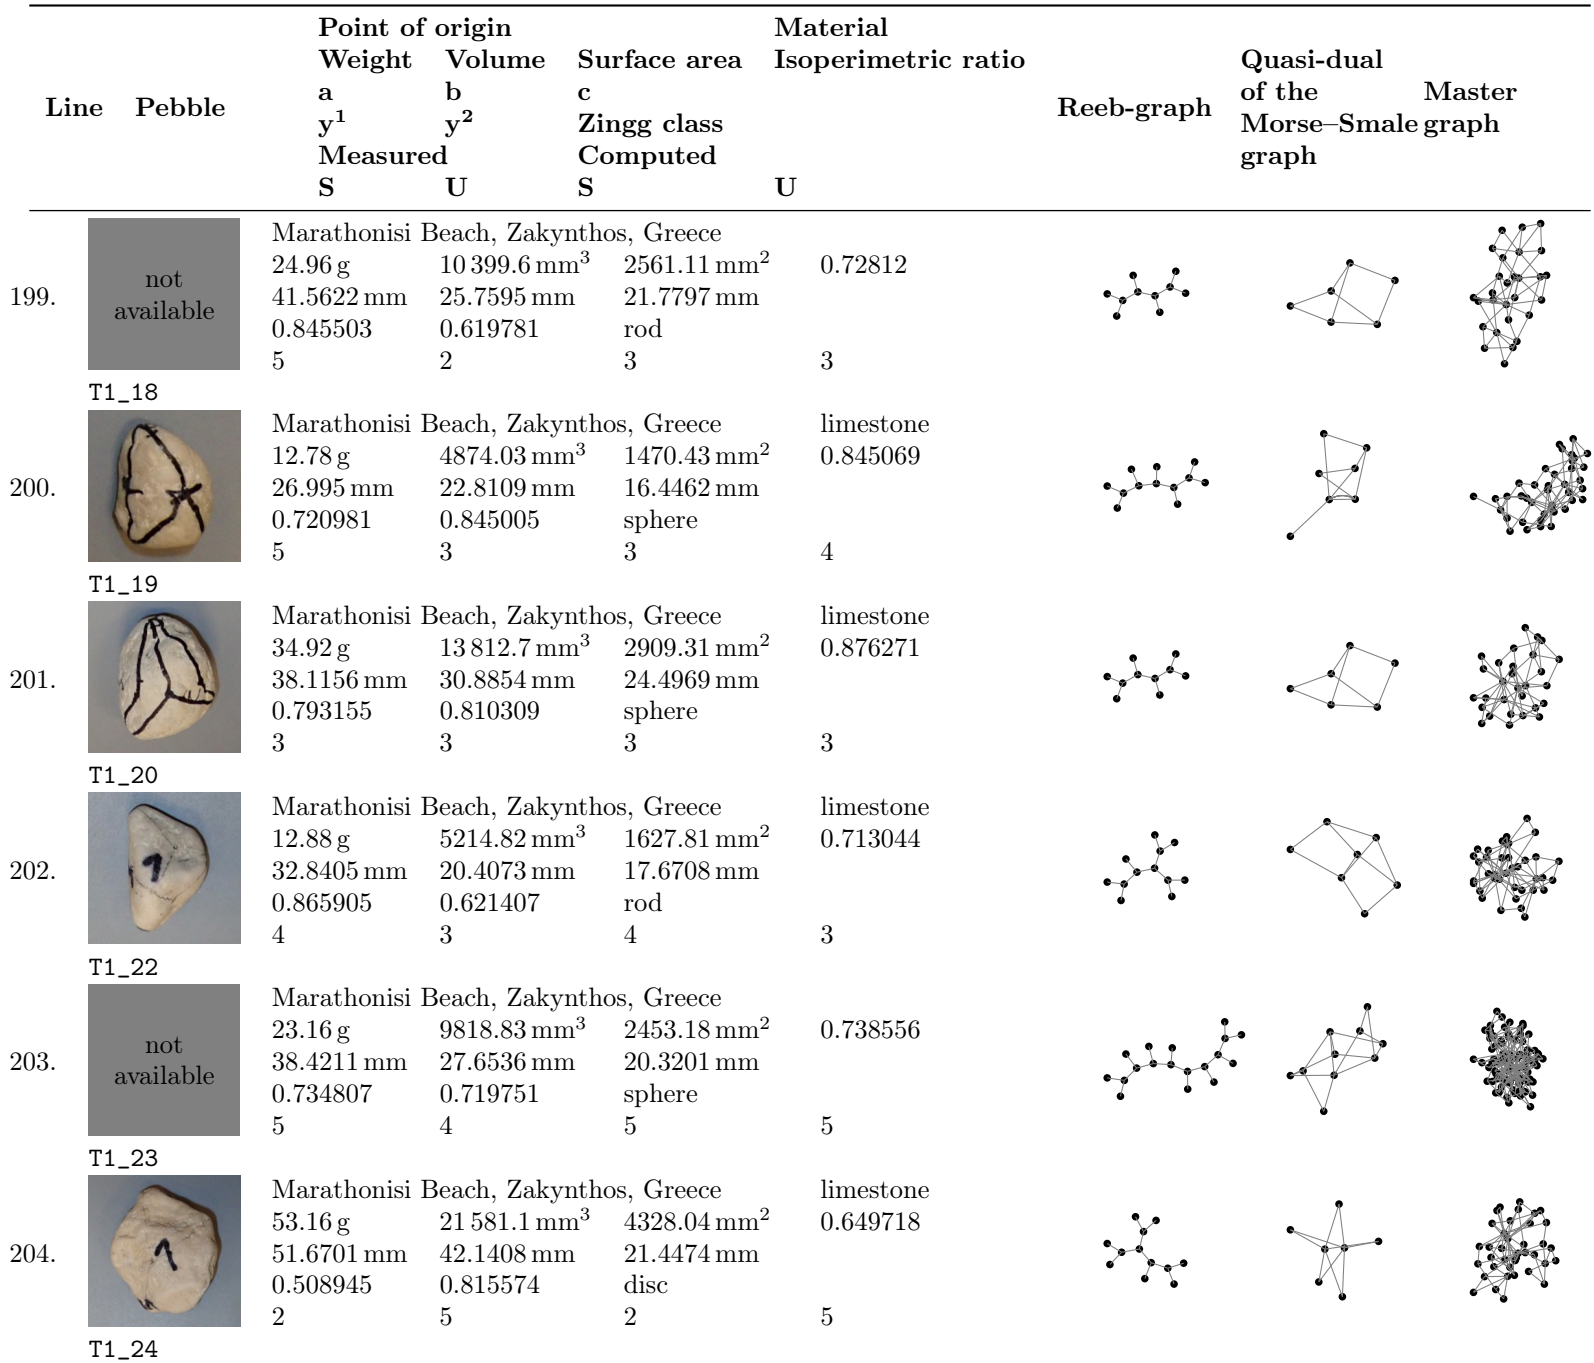 | 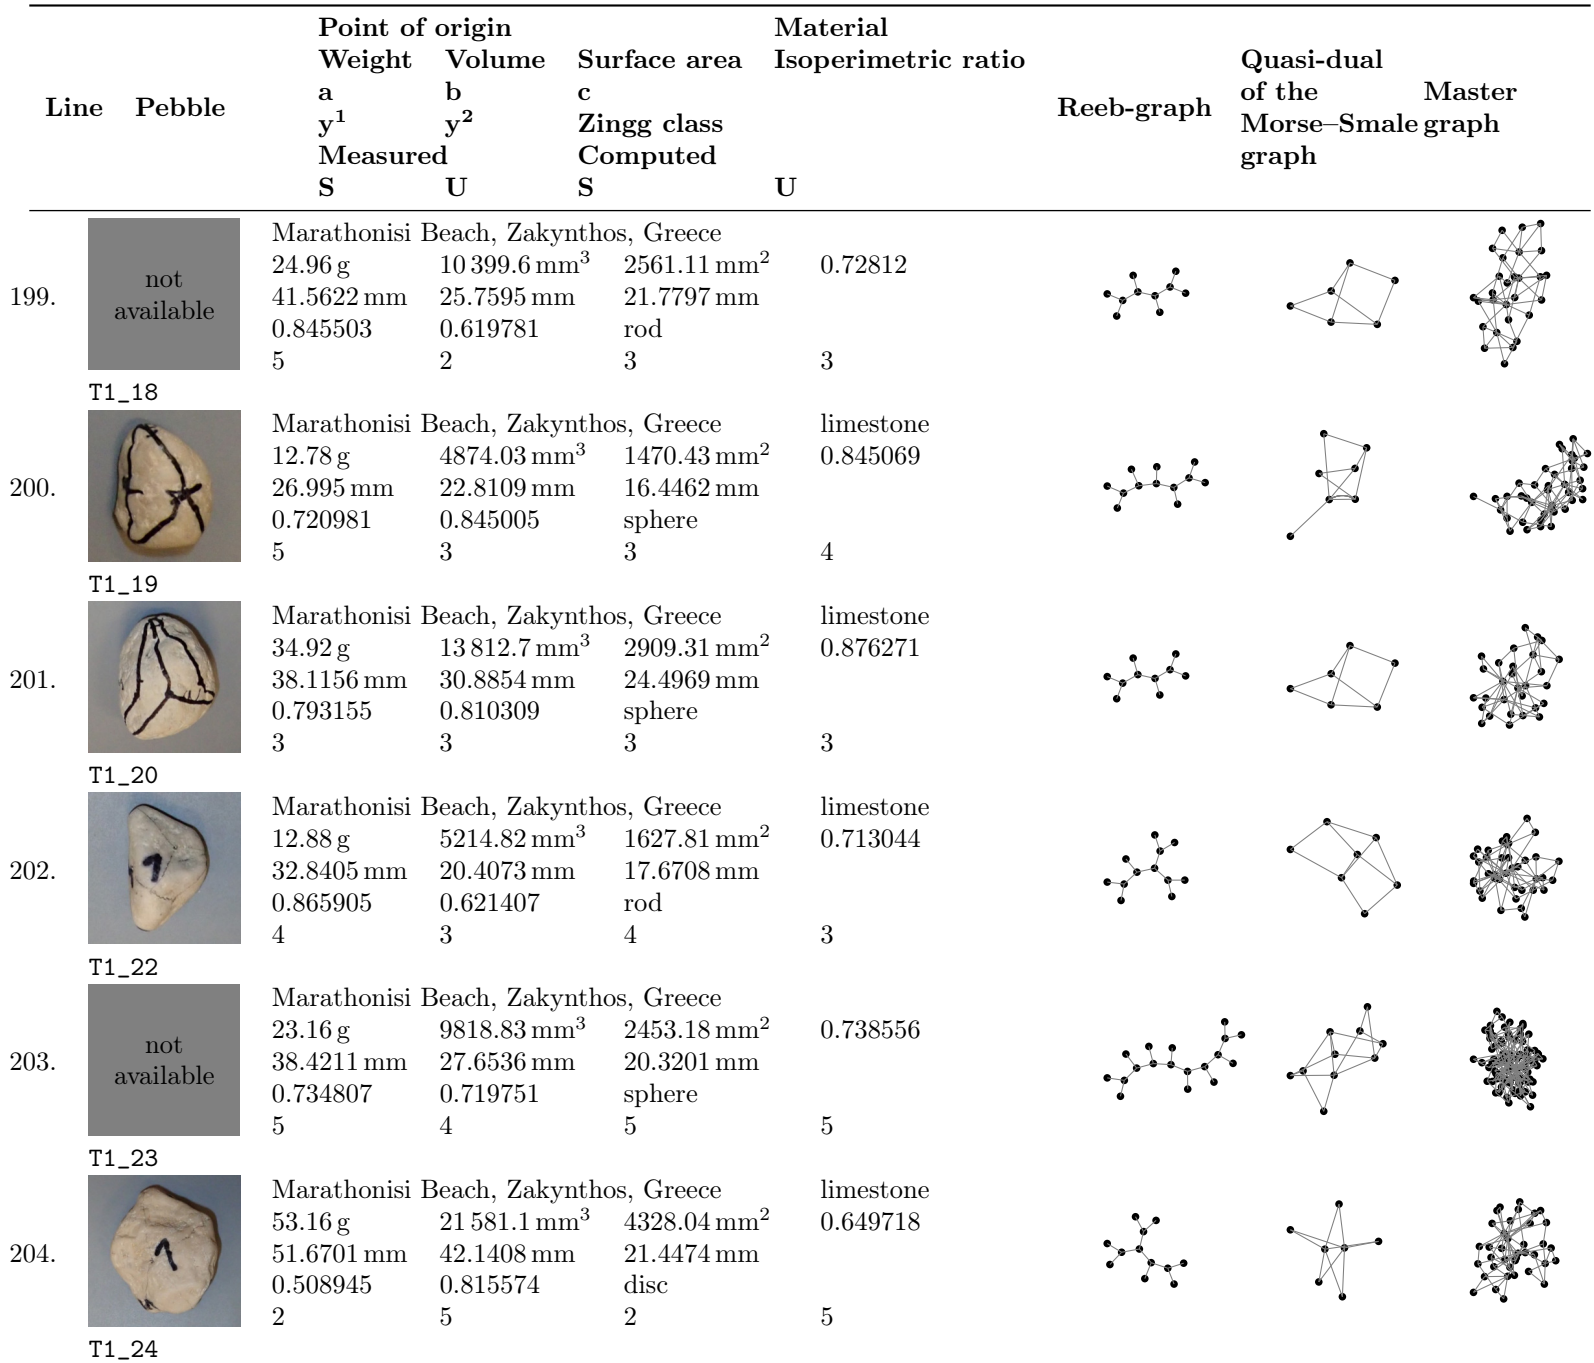 | 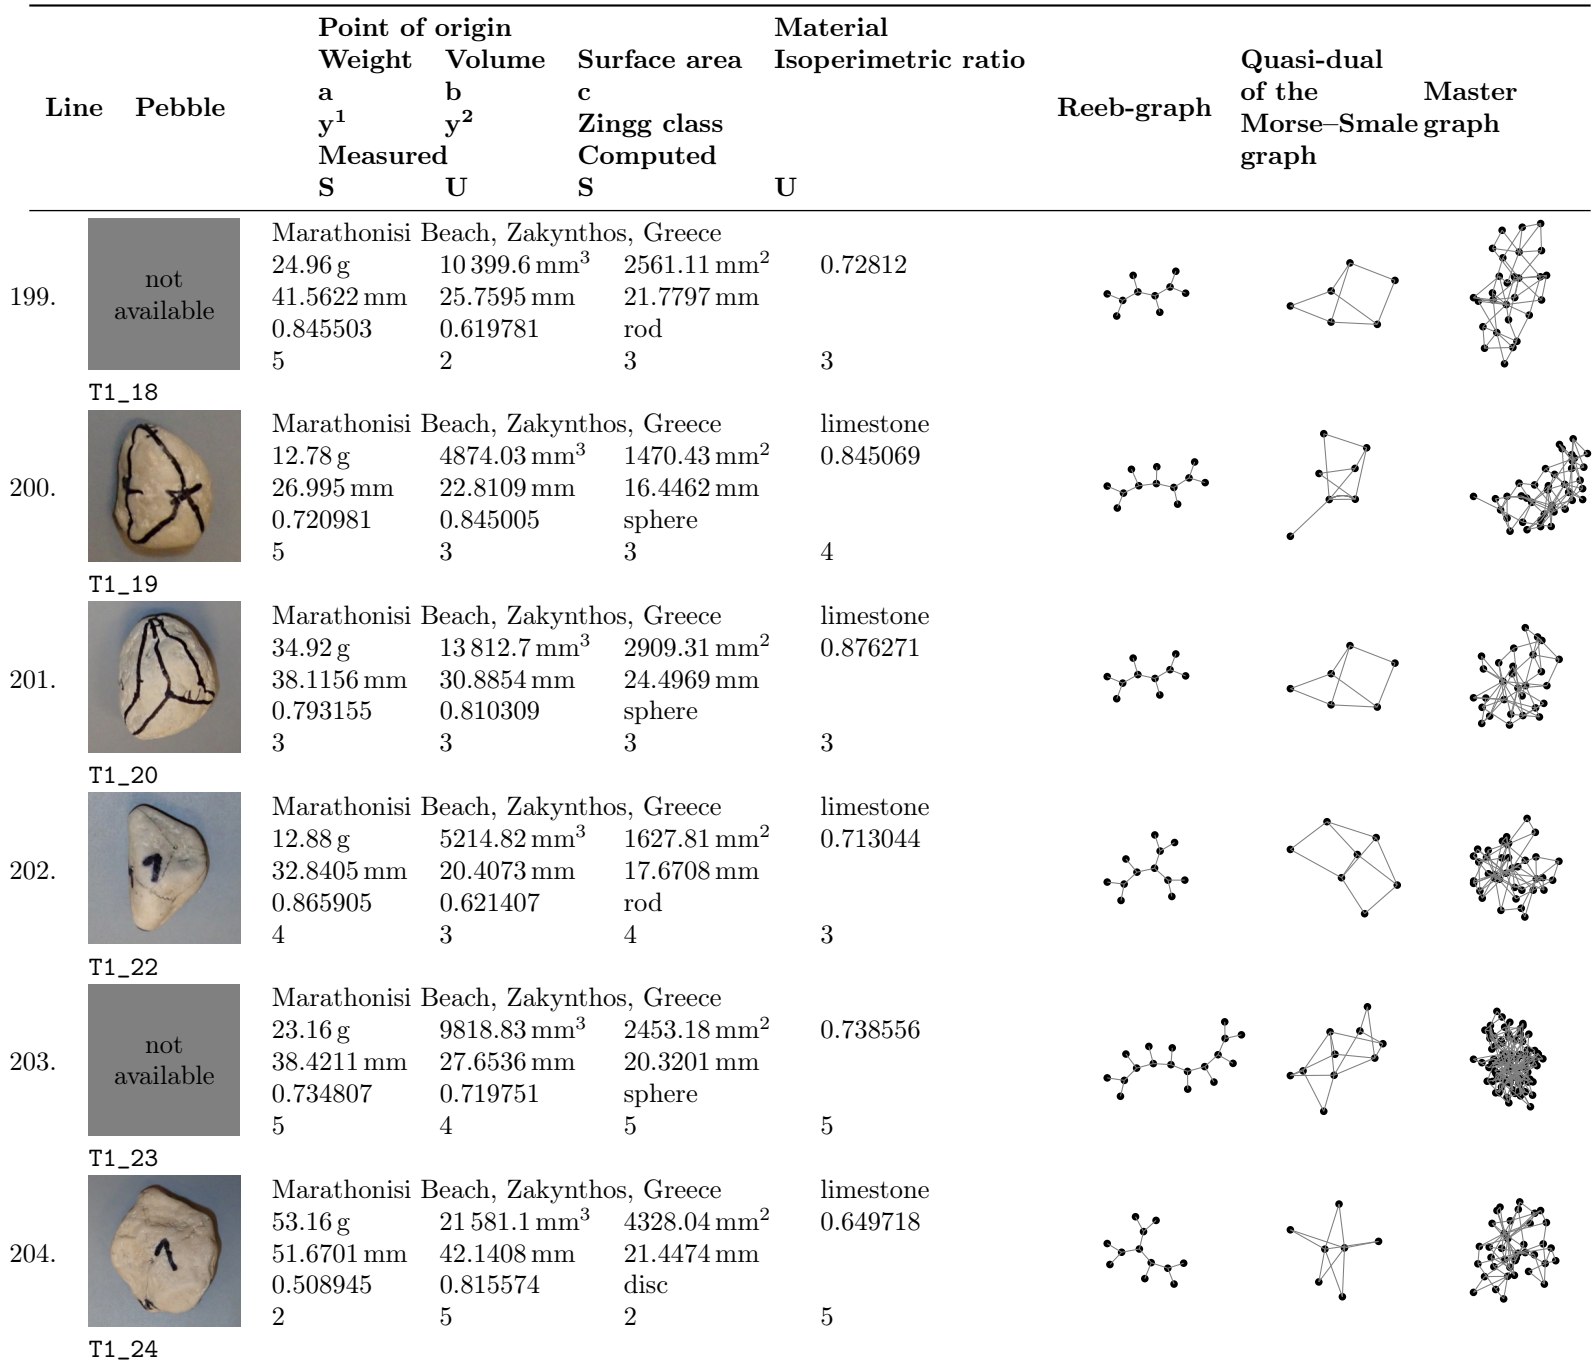 |
|      | T1_24                                                                               |                                                                                |                                                                    |                                                      |                                      |                                                                                       |                                                                                       |                                                                                       |

| Line | Pebble                                                                              | Point of origin                                                                |                                                         | Surface area<br>c<br>Zingg class<br>Computed<br>S    | Material<br>Isoperimetric ratio<br>U | Reeb-graph                                                                            | Quasi-dual<br>of the<br>Morse–Smale<br>graph                                          | Master<br>graph                                                                       |
|------|-------------------------------------------------------------------------------------|--------------------------------------------------------------------------------|---------------------------------------------------------|------------------------------------------------------|--------------------------------------|---------------------------------------------------------------------------------------|---------------------------------------------------------------------------------------|---------------------------------------------------------------------------------------|
|      |                                                                                     | Weight                                                                         | Volume                                                  |                                                      |                                      |                                                                                       |                                                                                       |                                                                                       |
|      |                                                                                     | a<br>y <sup>1</sup><br>Measured<br>S                                           | b<br>y <sup>2</sup><br>U                                |                                                      |                                      |                                                                                       |                                                                                       |                                                                                       |
|      |                                                                                     |                                                                                |                                                         |                                                      |                                      |                                                                                       |                                                                                       |                                                                                       |
| 205. | 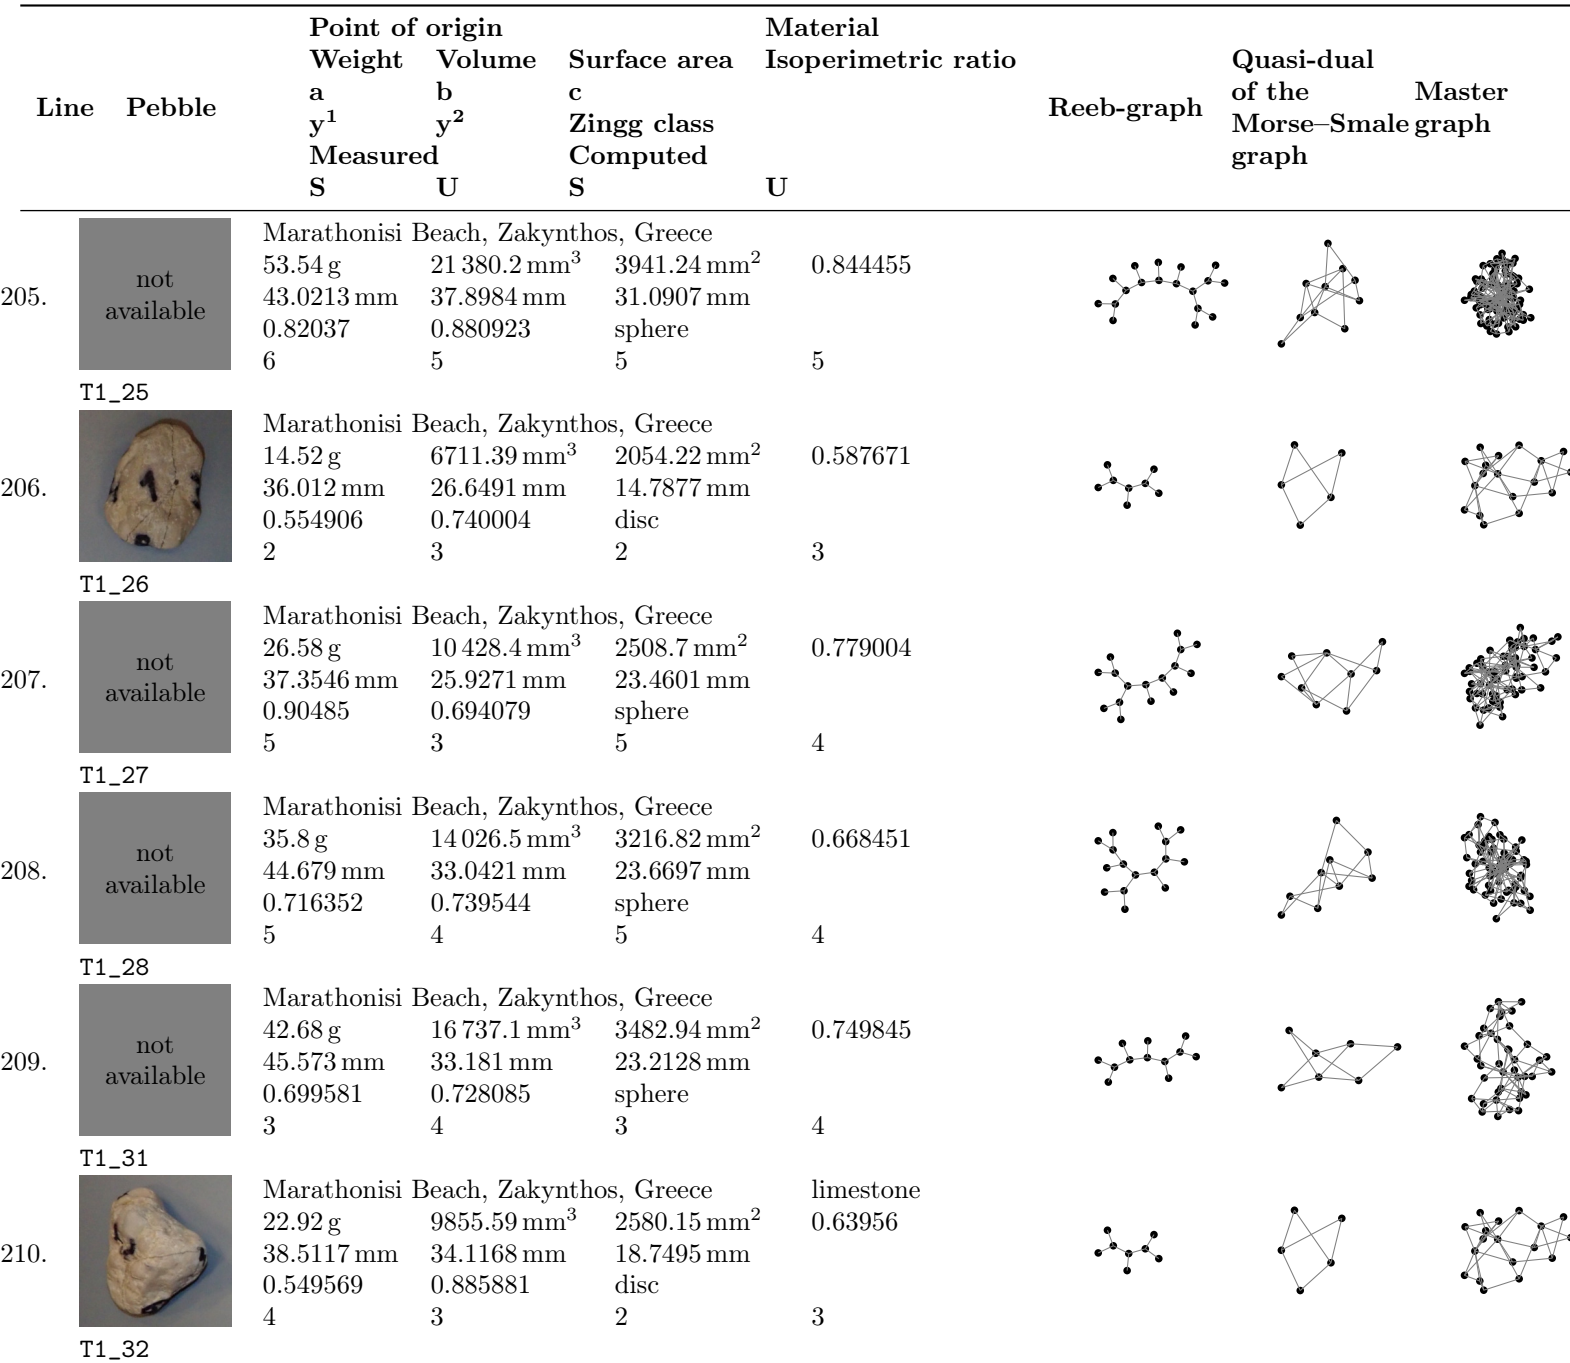   | Marathonisi Beach, Zakynthos, Greece<br>53.54 g<br>43.0213 mm<br>0.82037<br>6  | 21 380.2 mm <sup>3</sup><br>37.8984 mm<br>0.880923<br>5 | 3941.24 mm <sup>2</sup><br>31.0907 mm<br>sphere<br>5 | 0.844455                             | 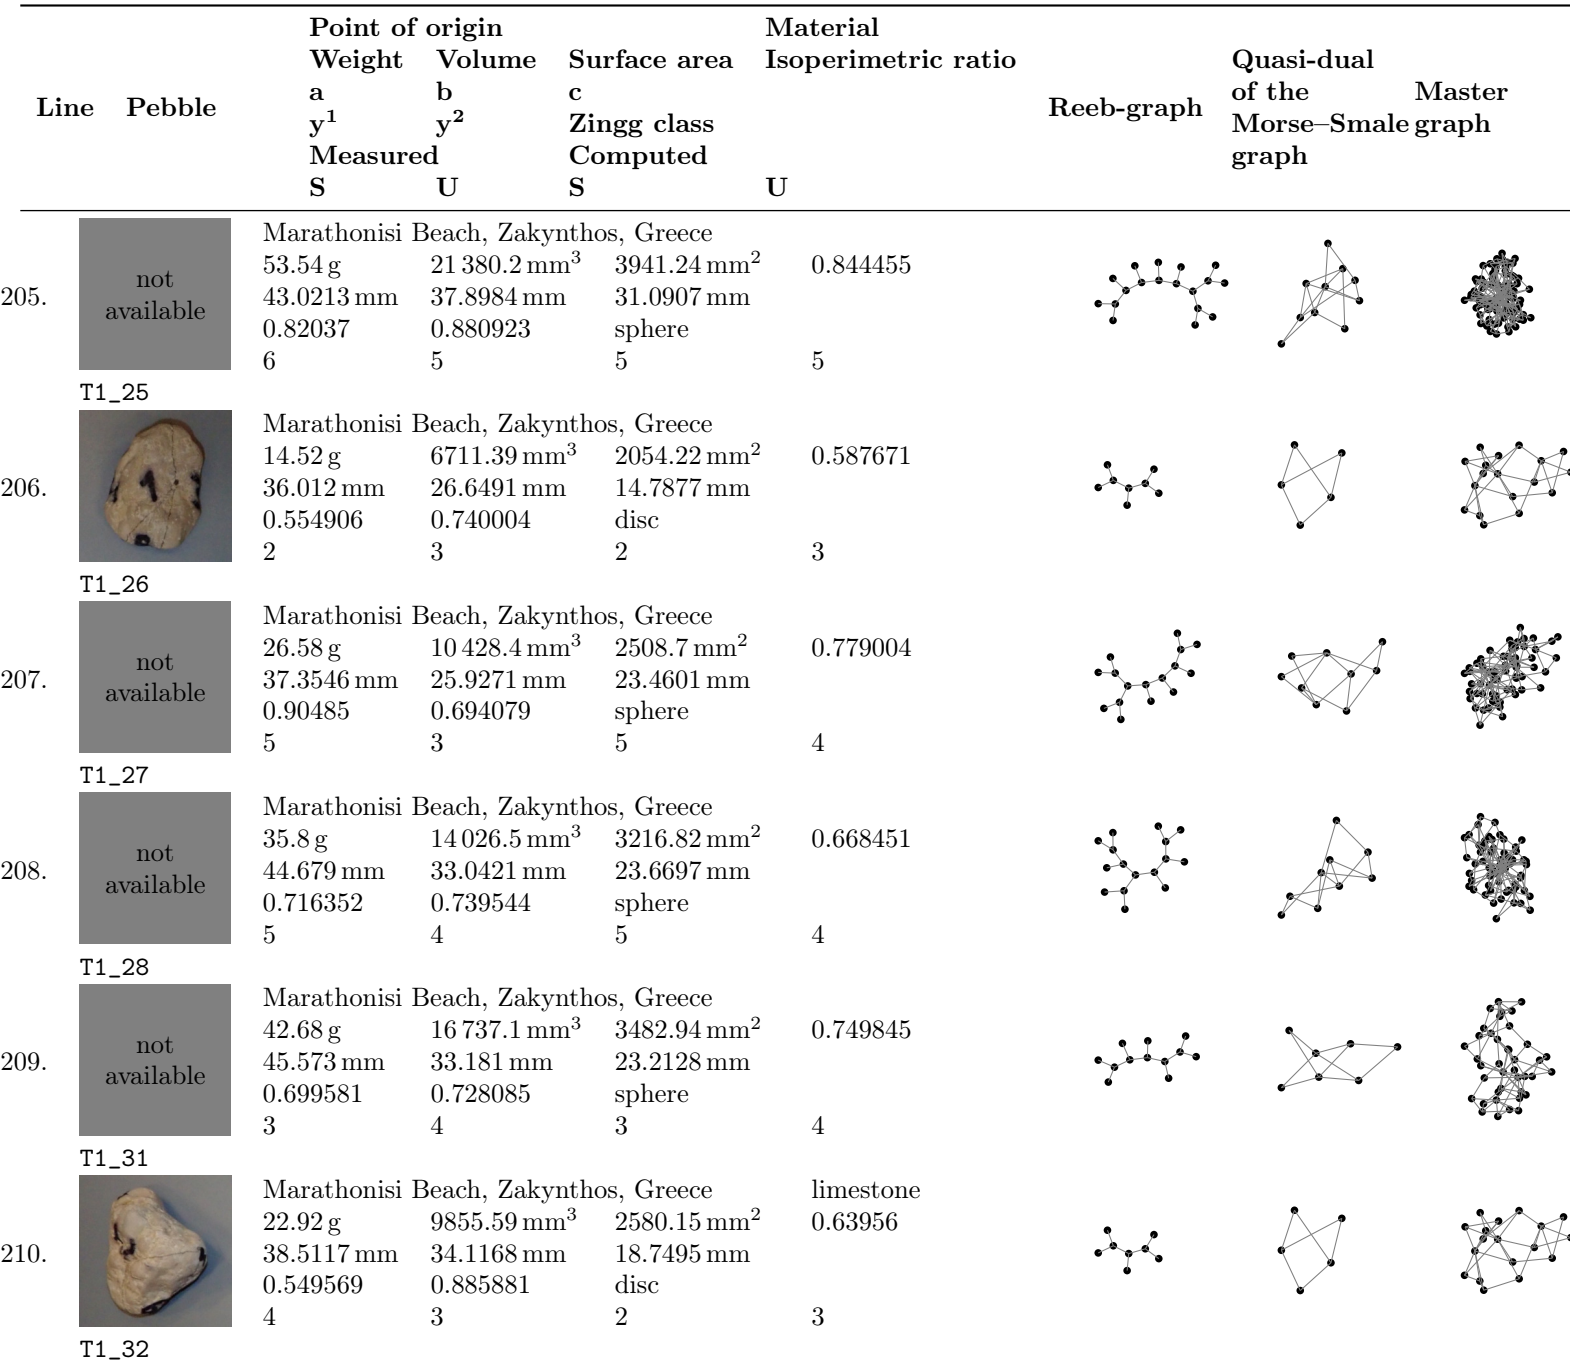   | 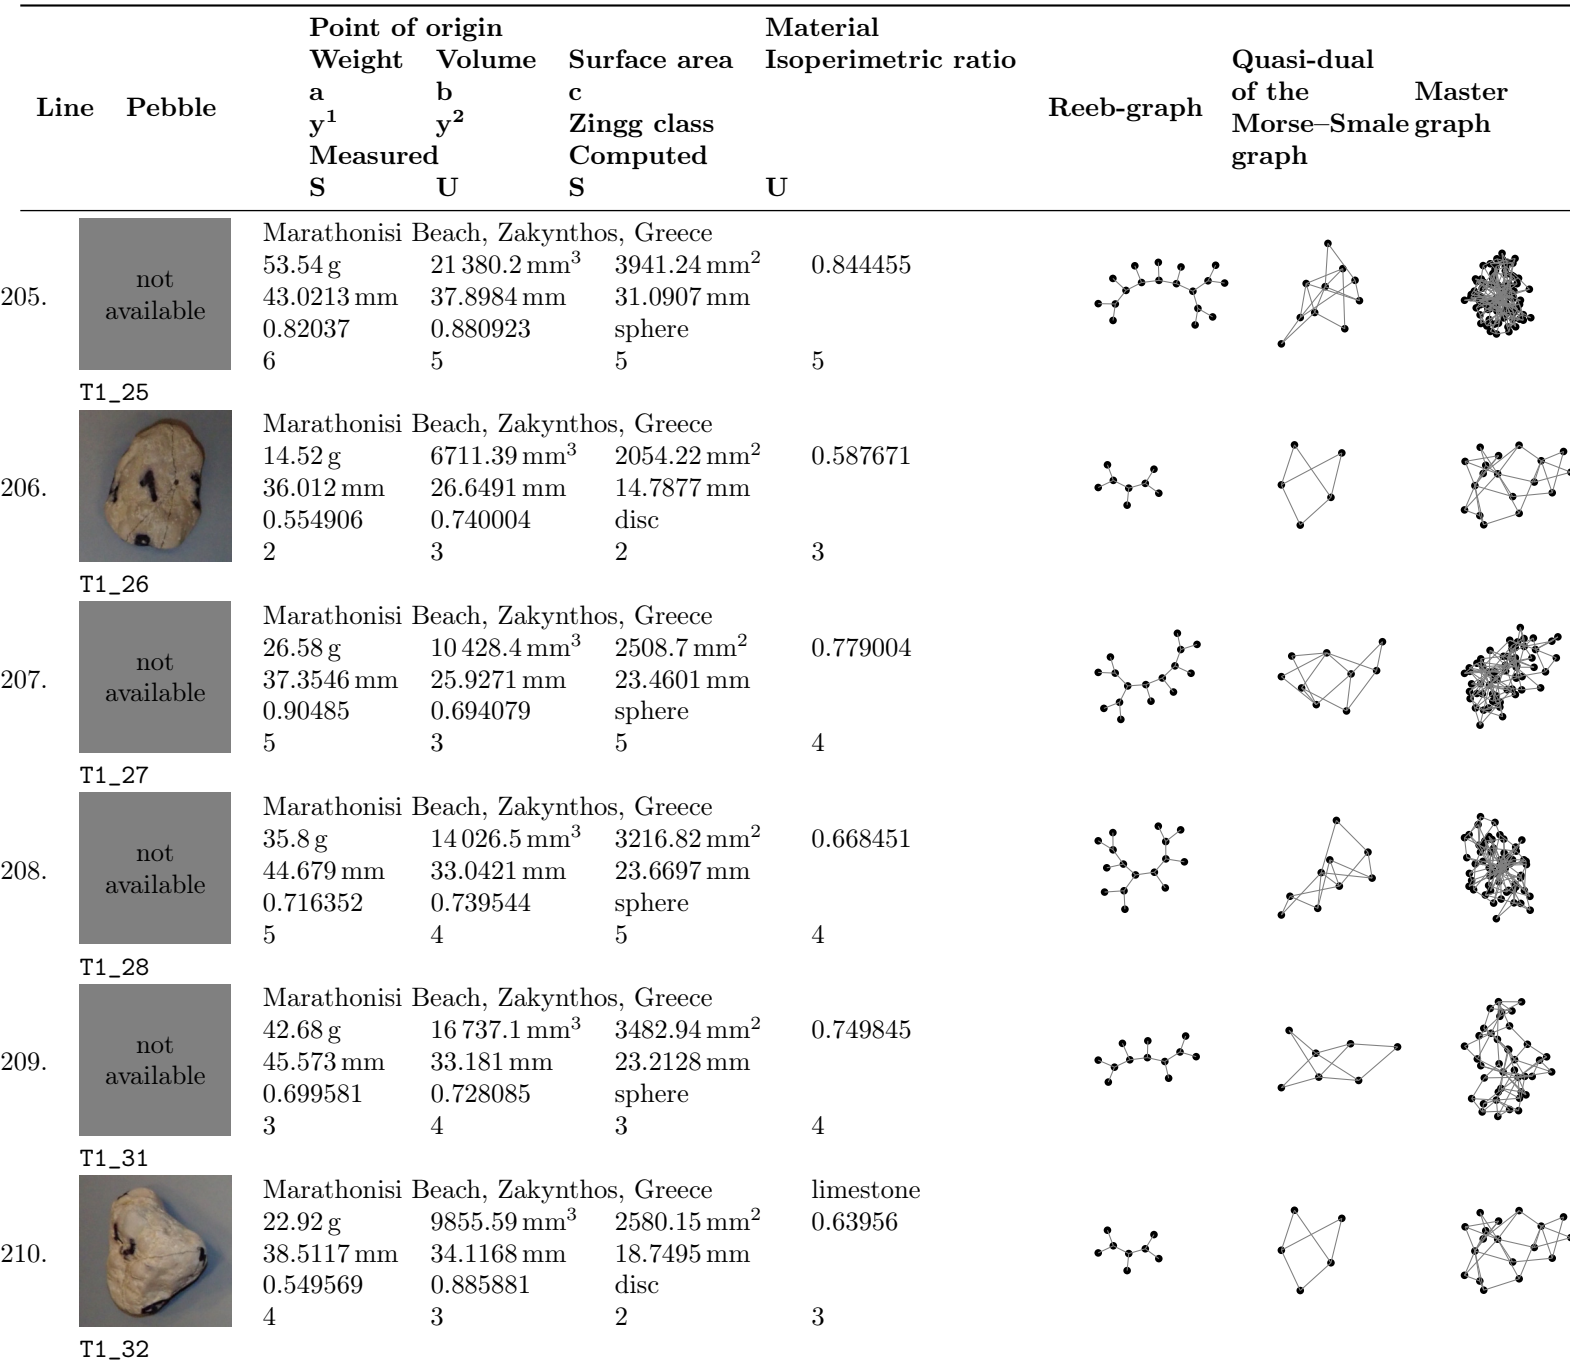   | 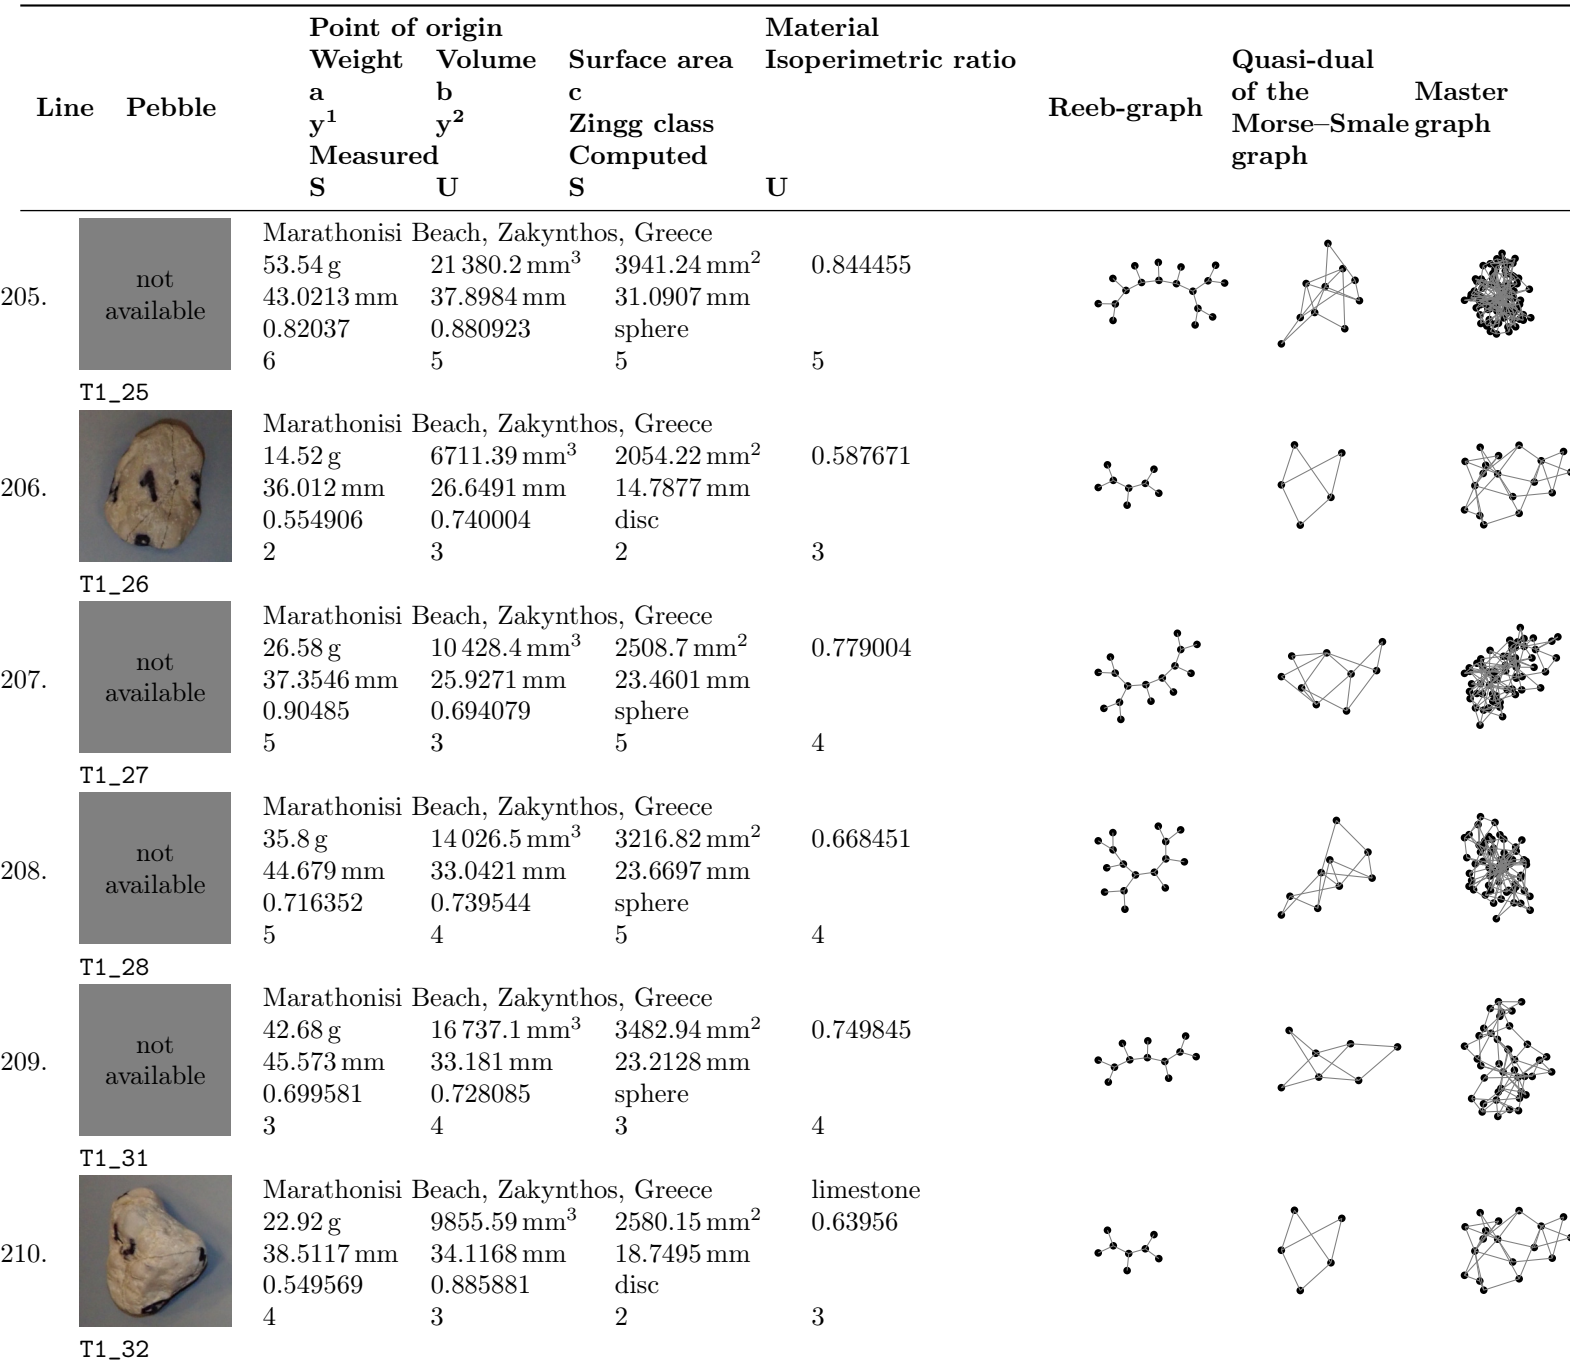   |
|      | T1_25                                                                               |                                                                                |                                                         |                                                      |                                      |                                                                                       |                                                                                       |                                                                                       |
| 206. | 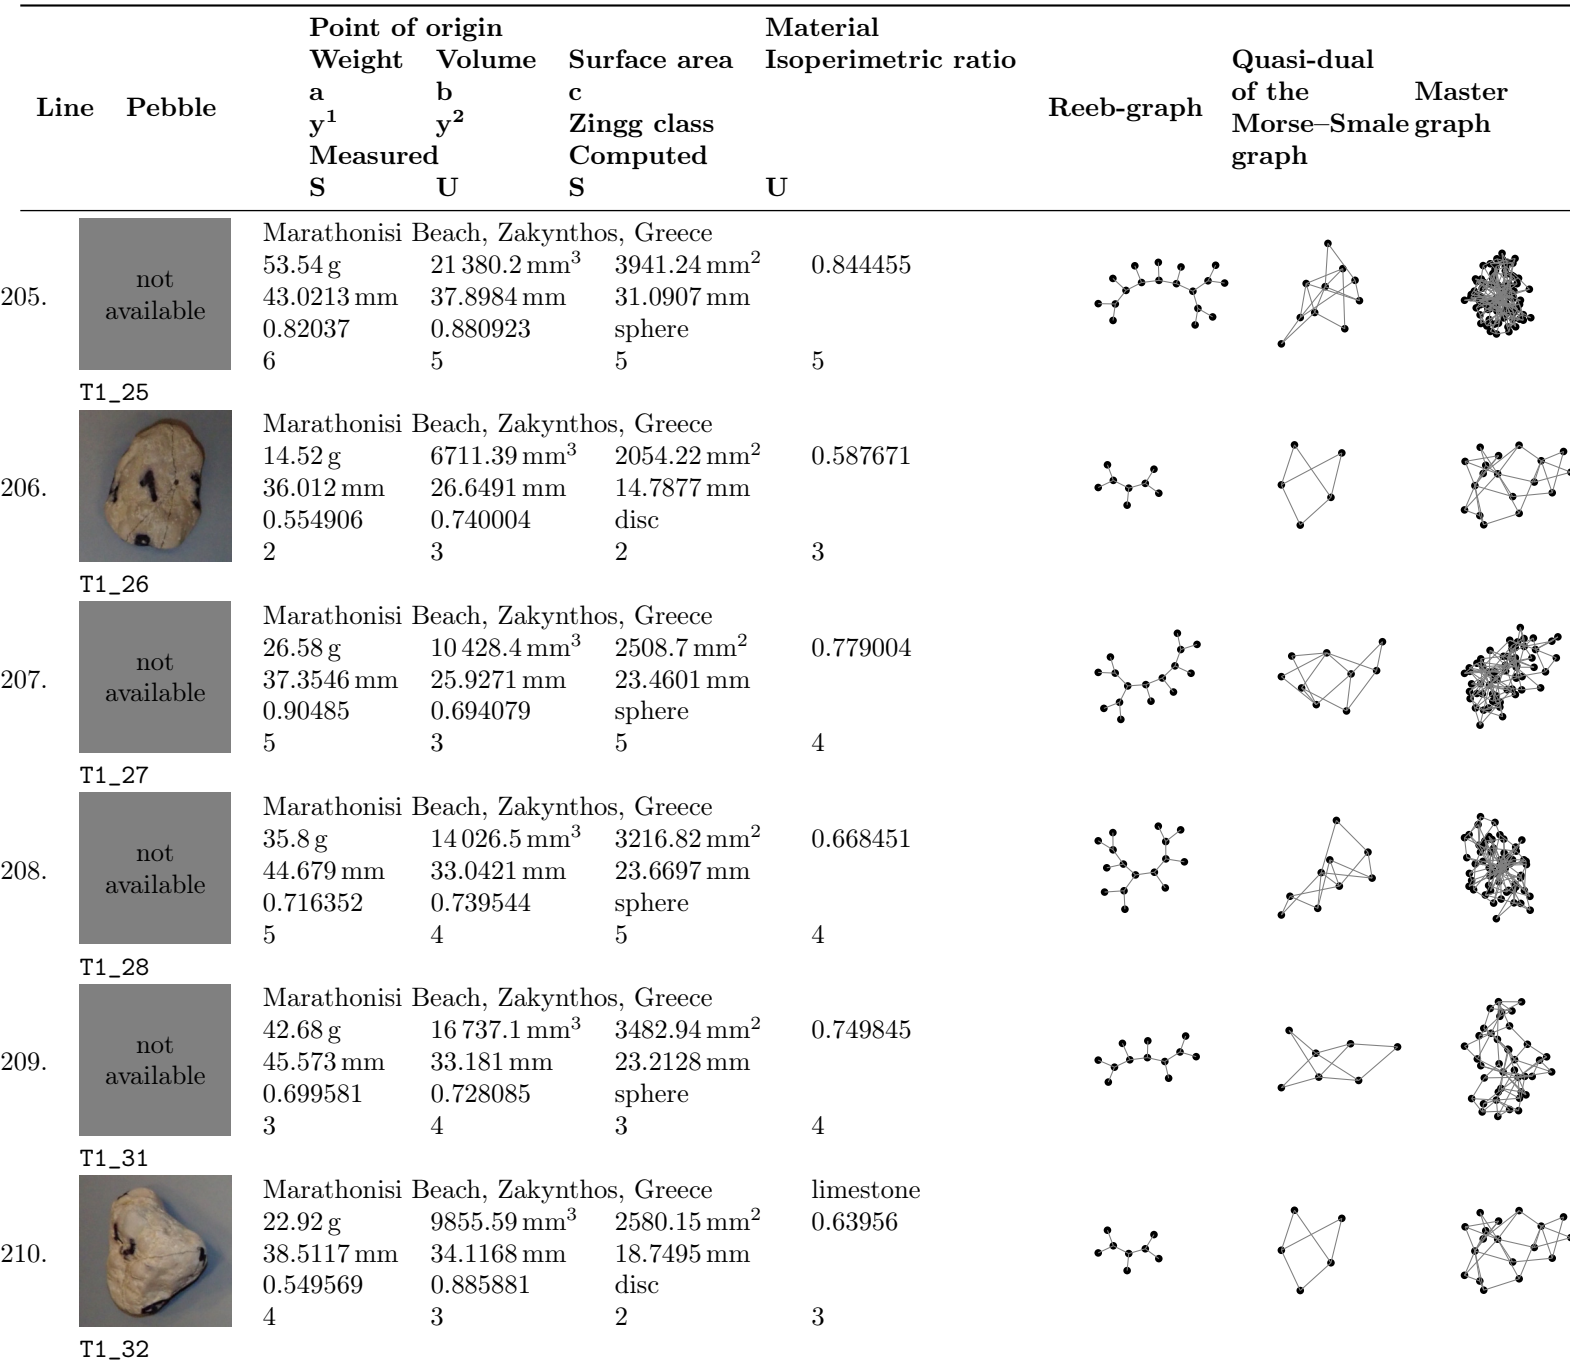   | Marathonisi Beach, Zakynthos, Greece<br>14.52 g<br>36.012 mm<br>0.554906<br>2  | 6711.39 mm <sup>3</sup><br>26.6491 mm<br>0.740004<br>3  | 2054.22 mm <sup>2</sup><br>14.7877 mm<br>disc<br>2   | 0.587671                             | 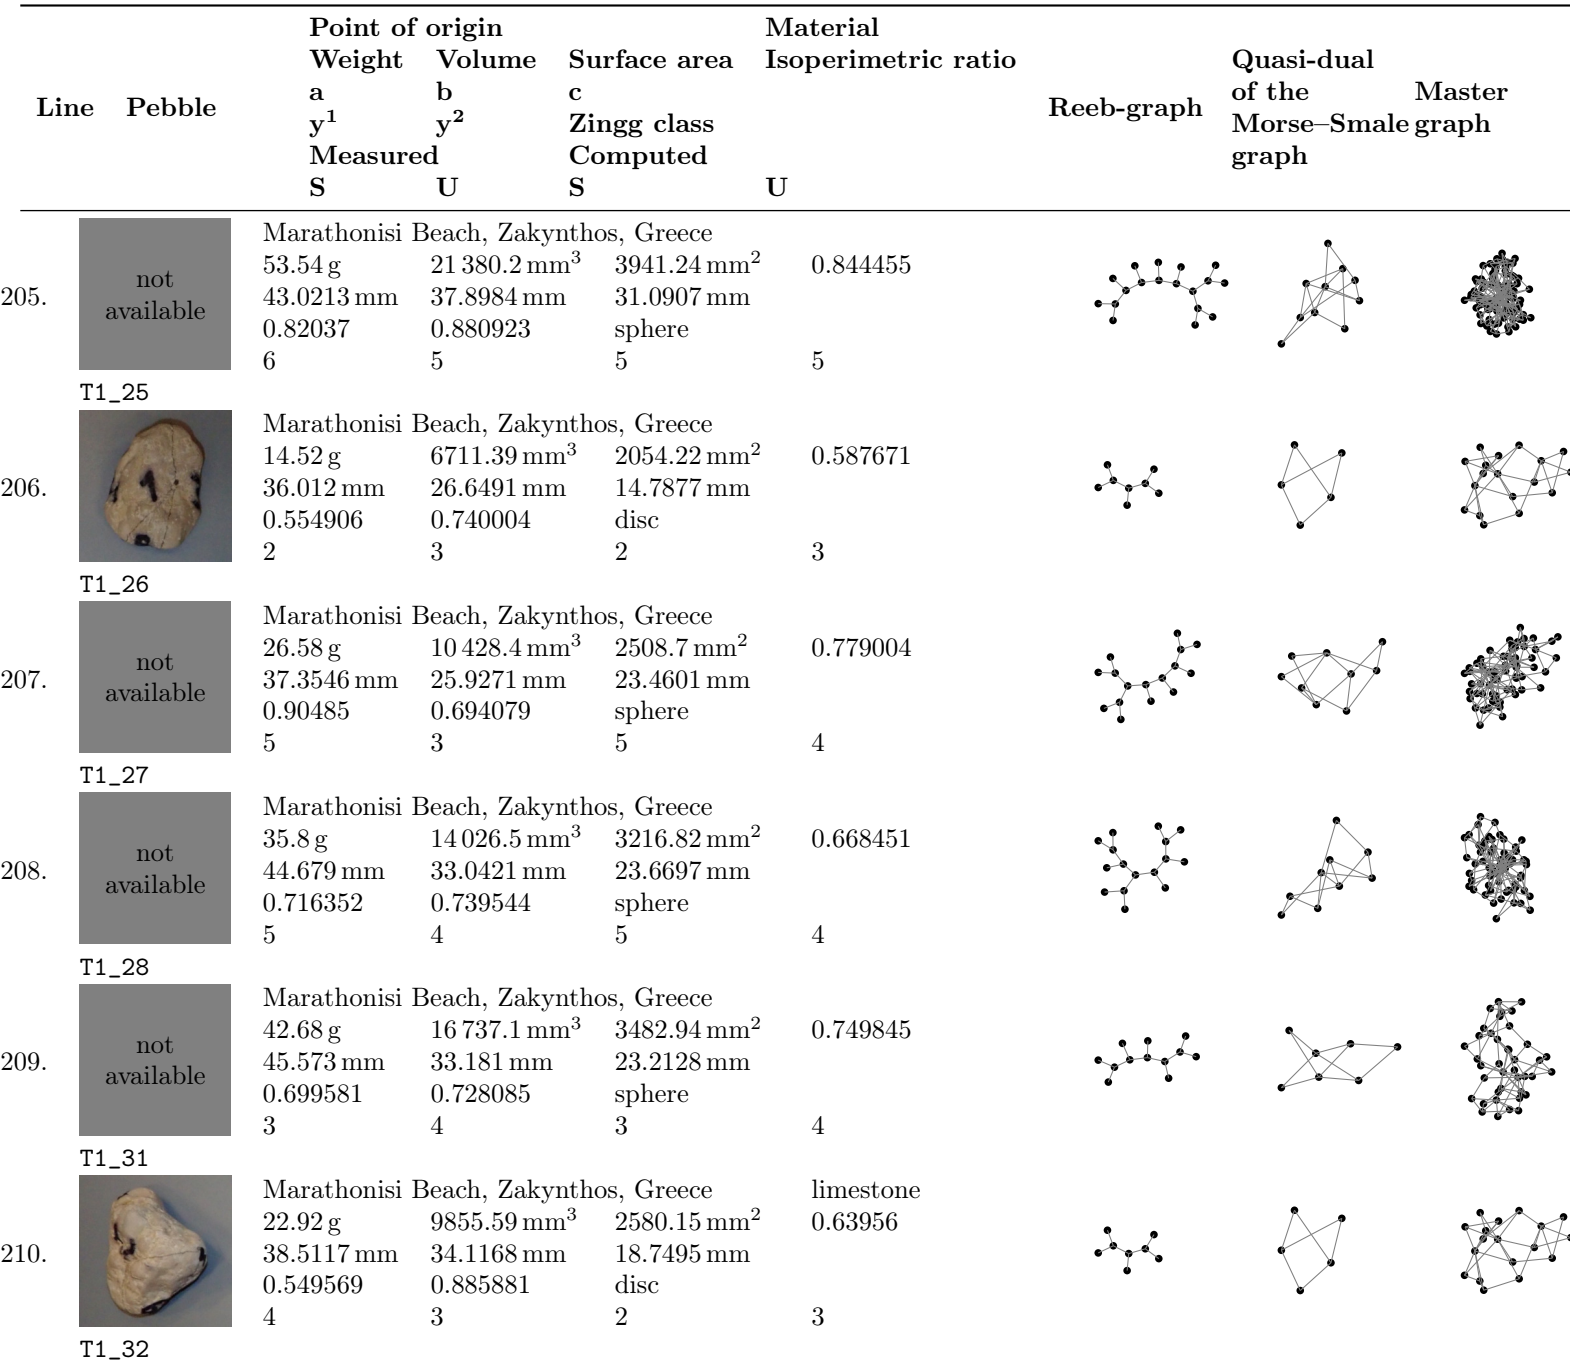   | 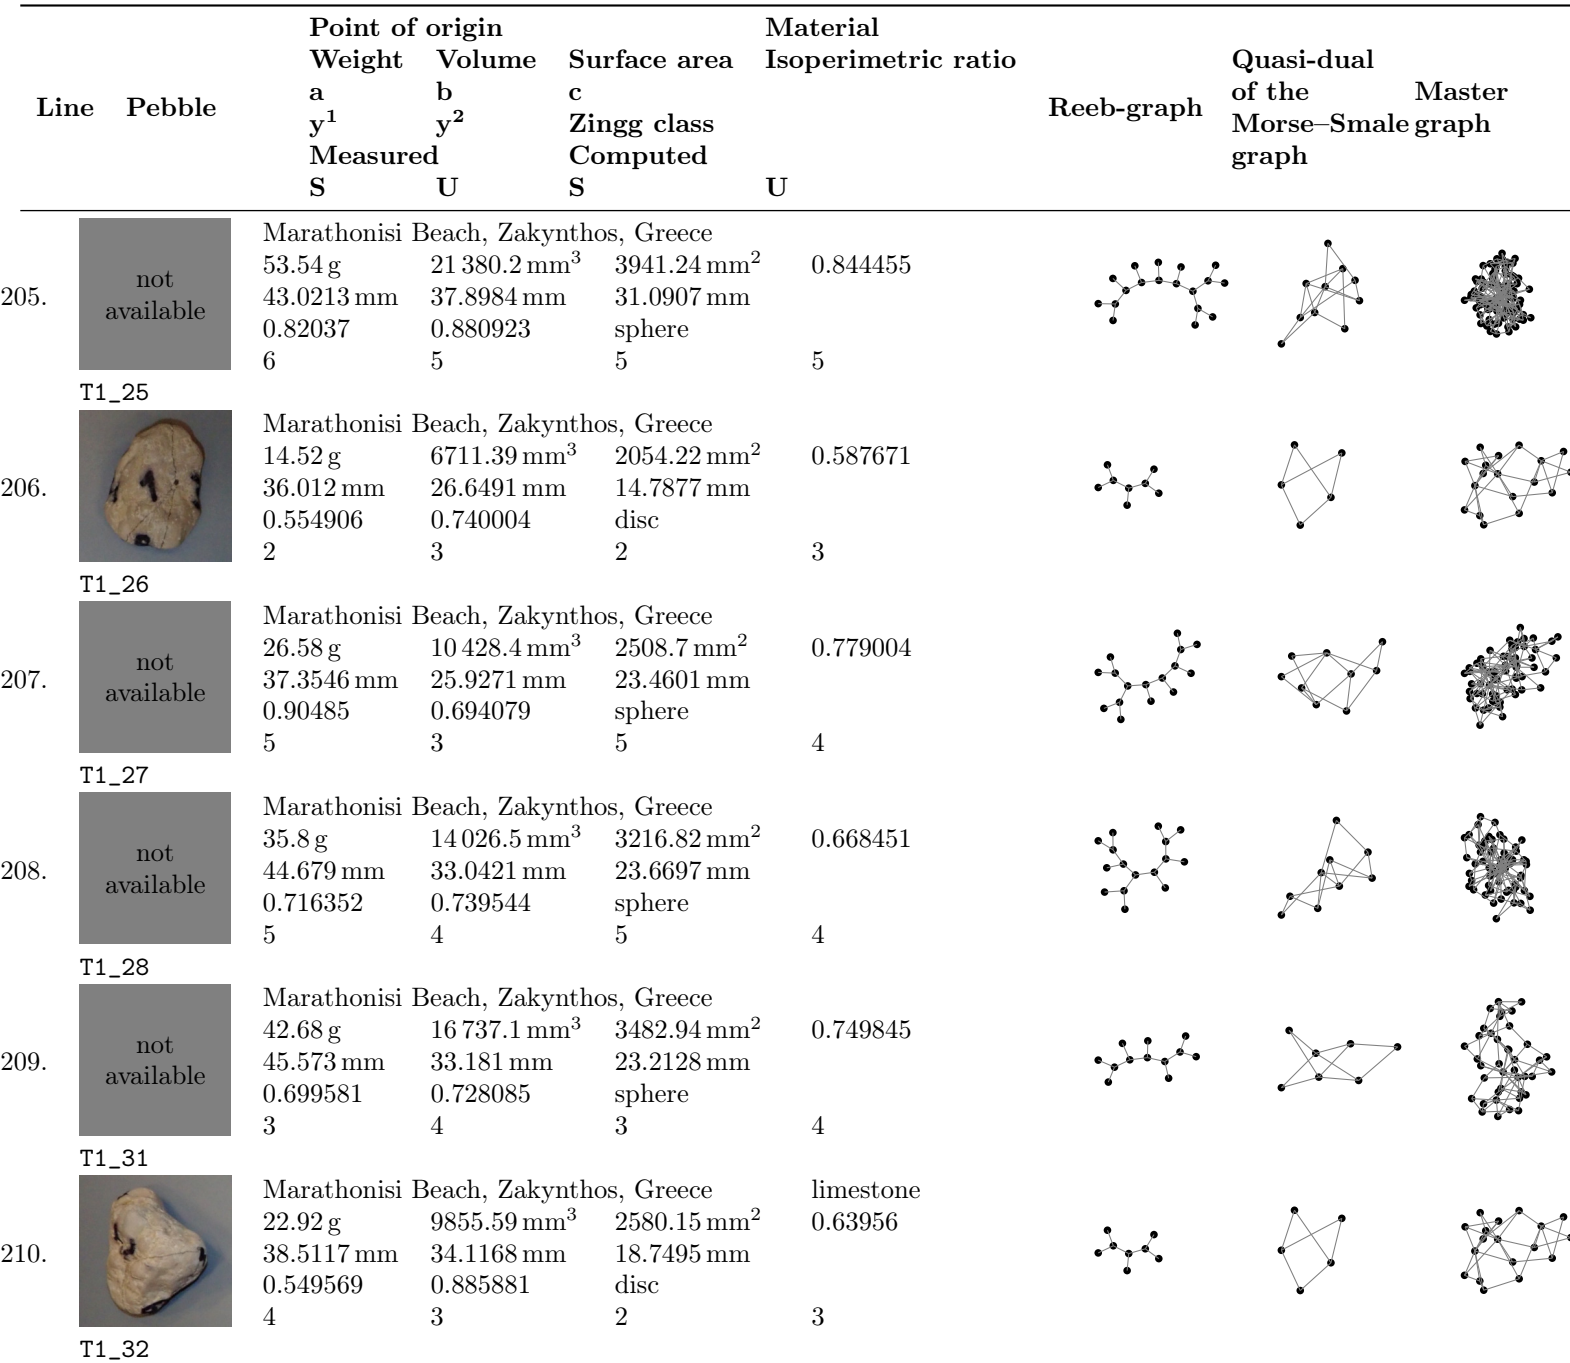   | 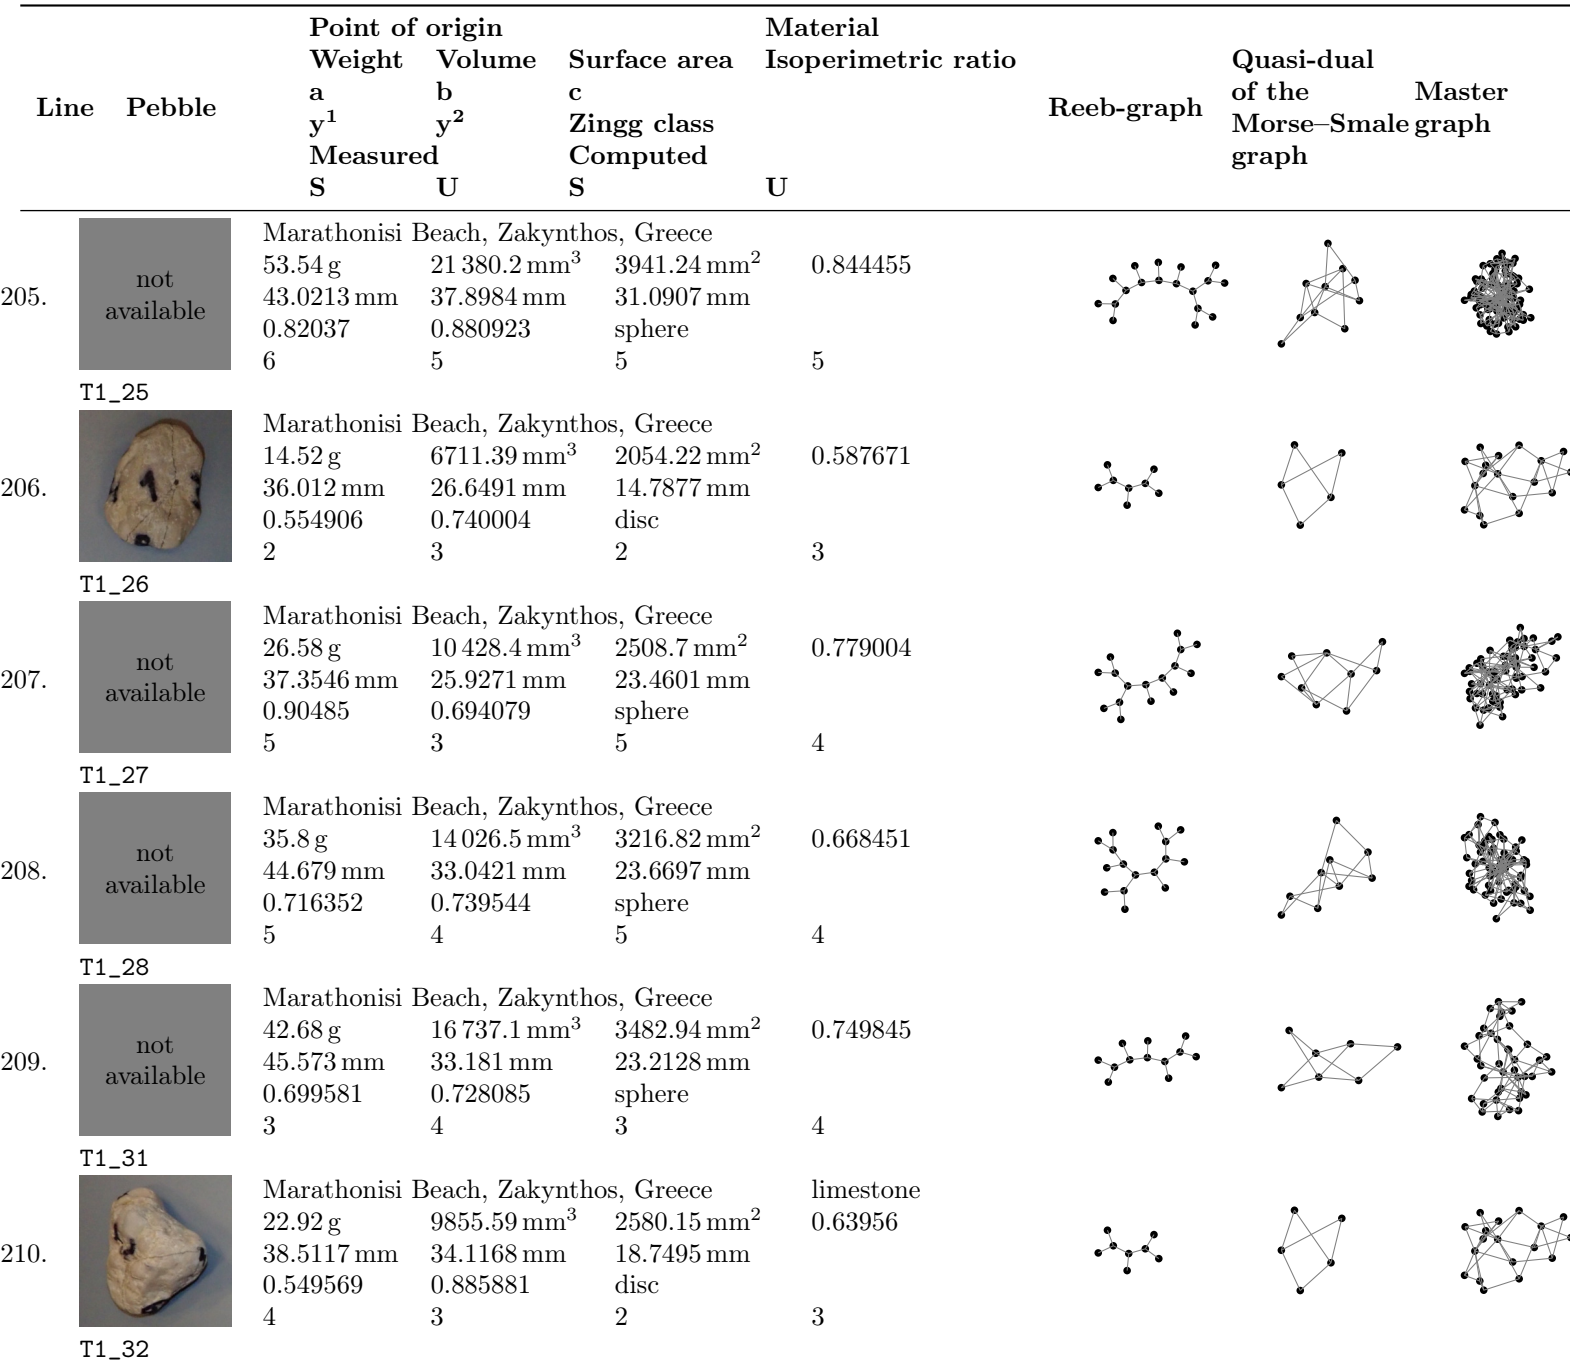   |
|      | T1_26                                                                               |                                                                                |                                                         |                                                      |                                      |                                                                                       |                                                                                       |                                                                                       |
| 207. | 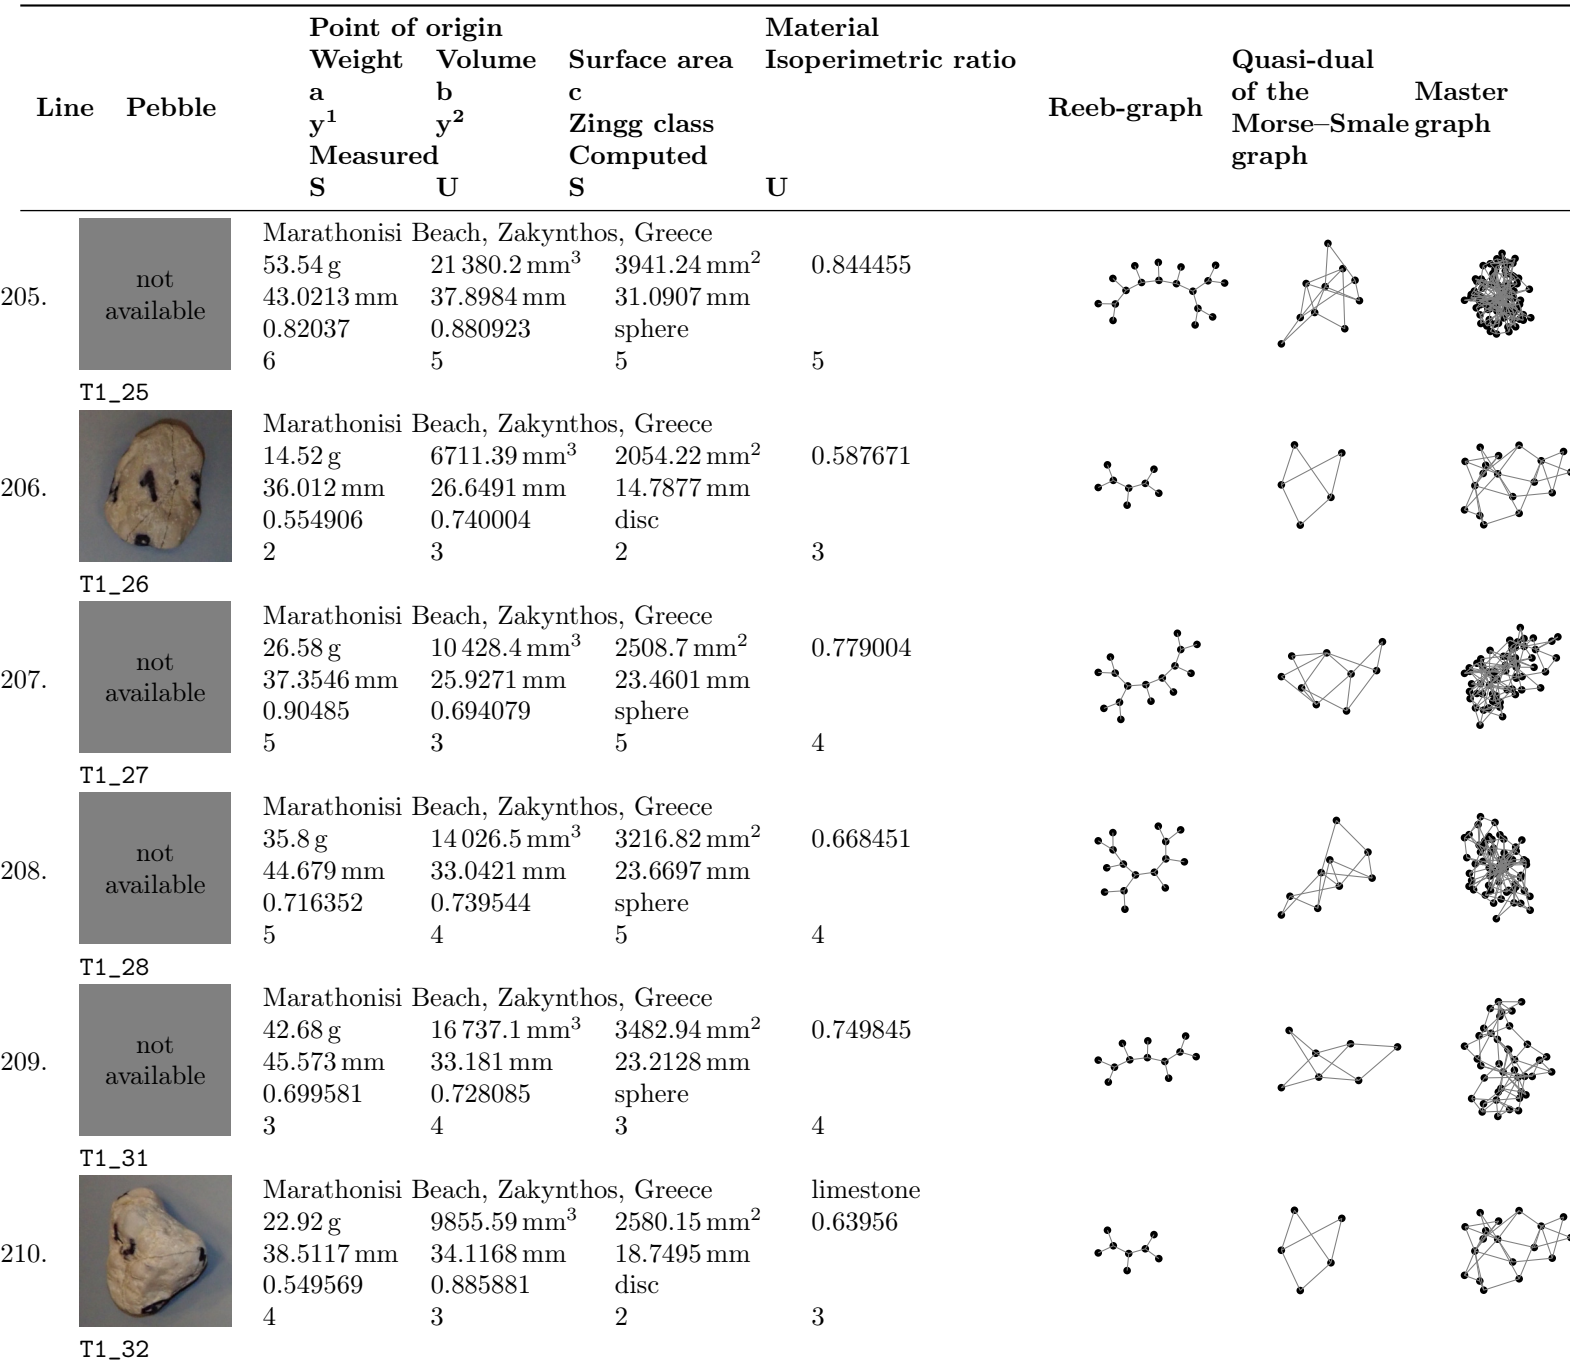   | Marathonisi Beach, Zakynthos, Greece<br>26.58 g<br>37.3546 mm<br>0.90485<br>5  | 10 428.4 mm <sup>3</sup><br>25.9271 mm<br>0.694079<br>3 | 2508.7 mm <sup>2</sup><br>23.4601 mm<br>sphere<br>5  | 0.779004                             | 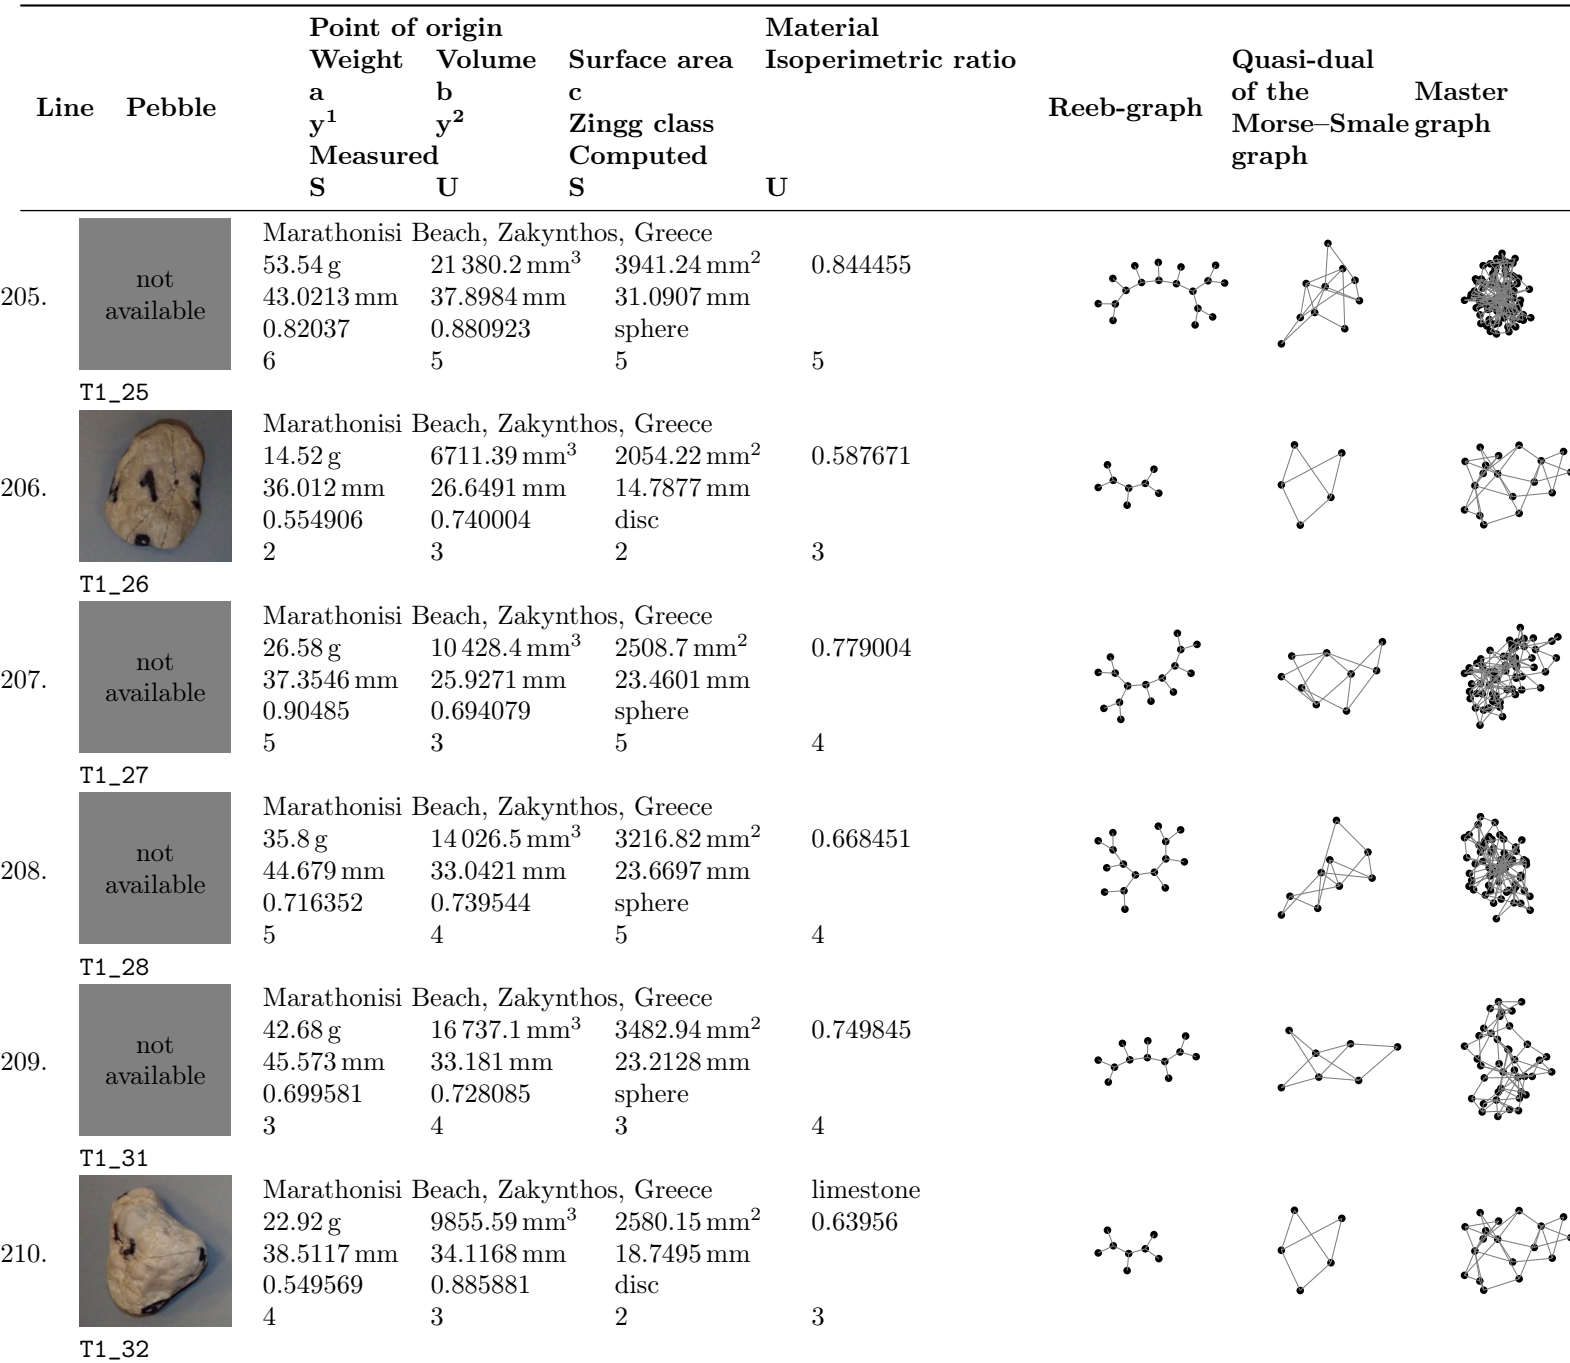   | 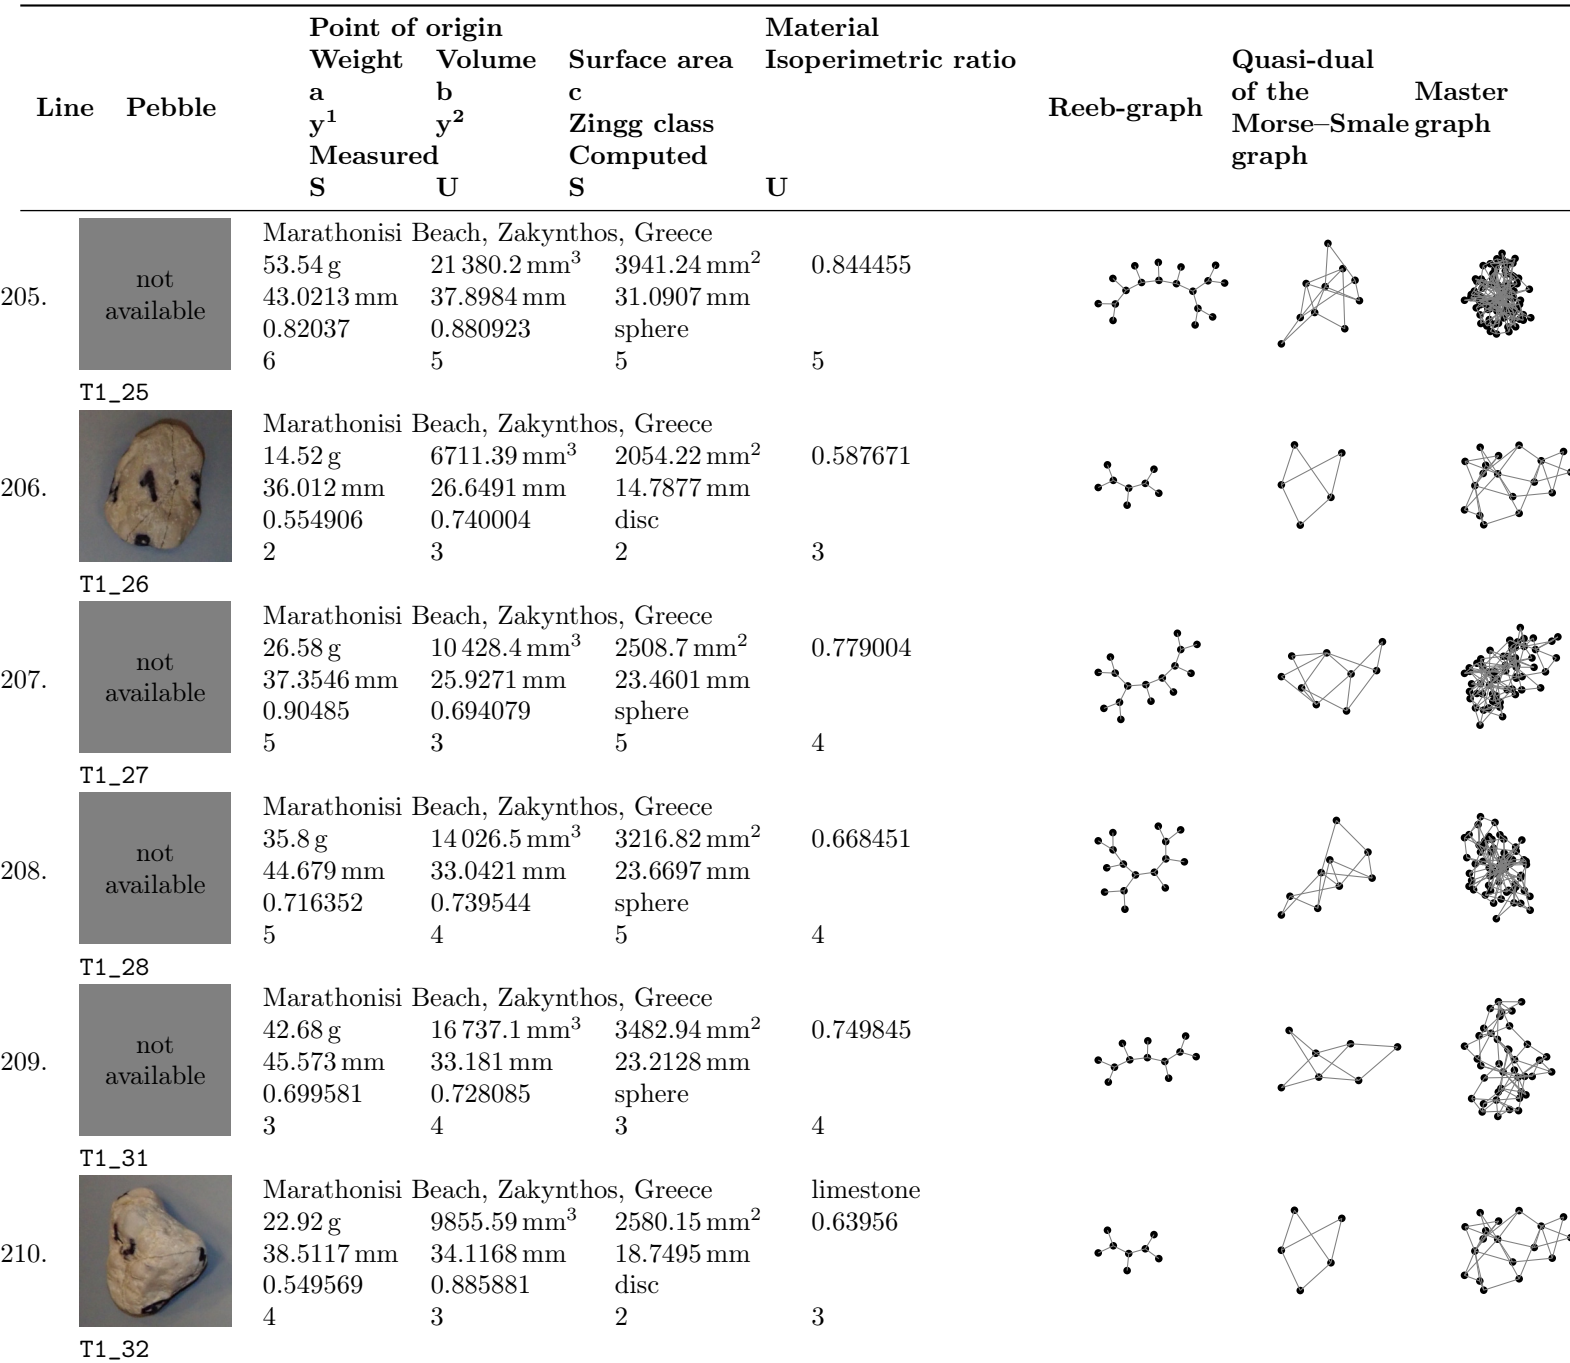   | 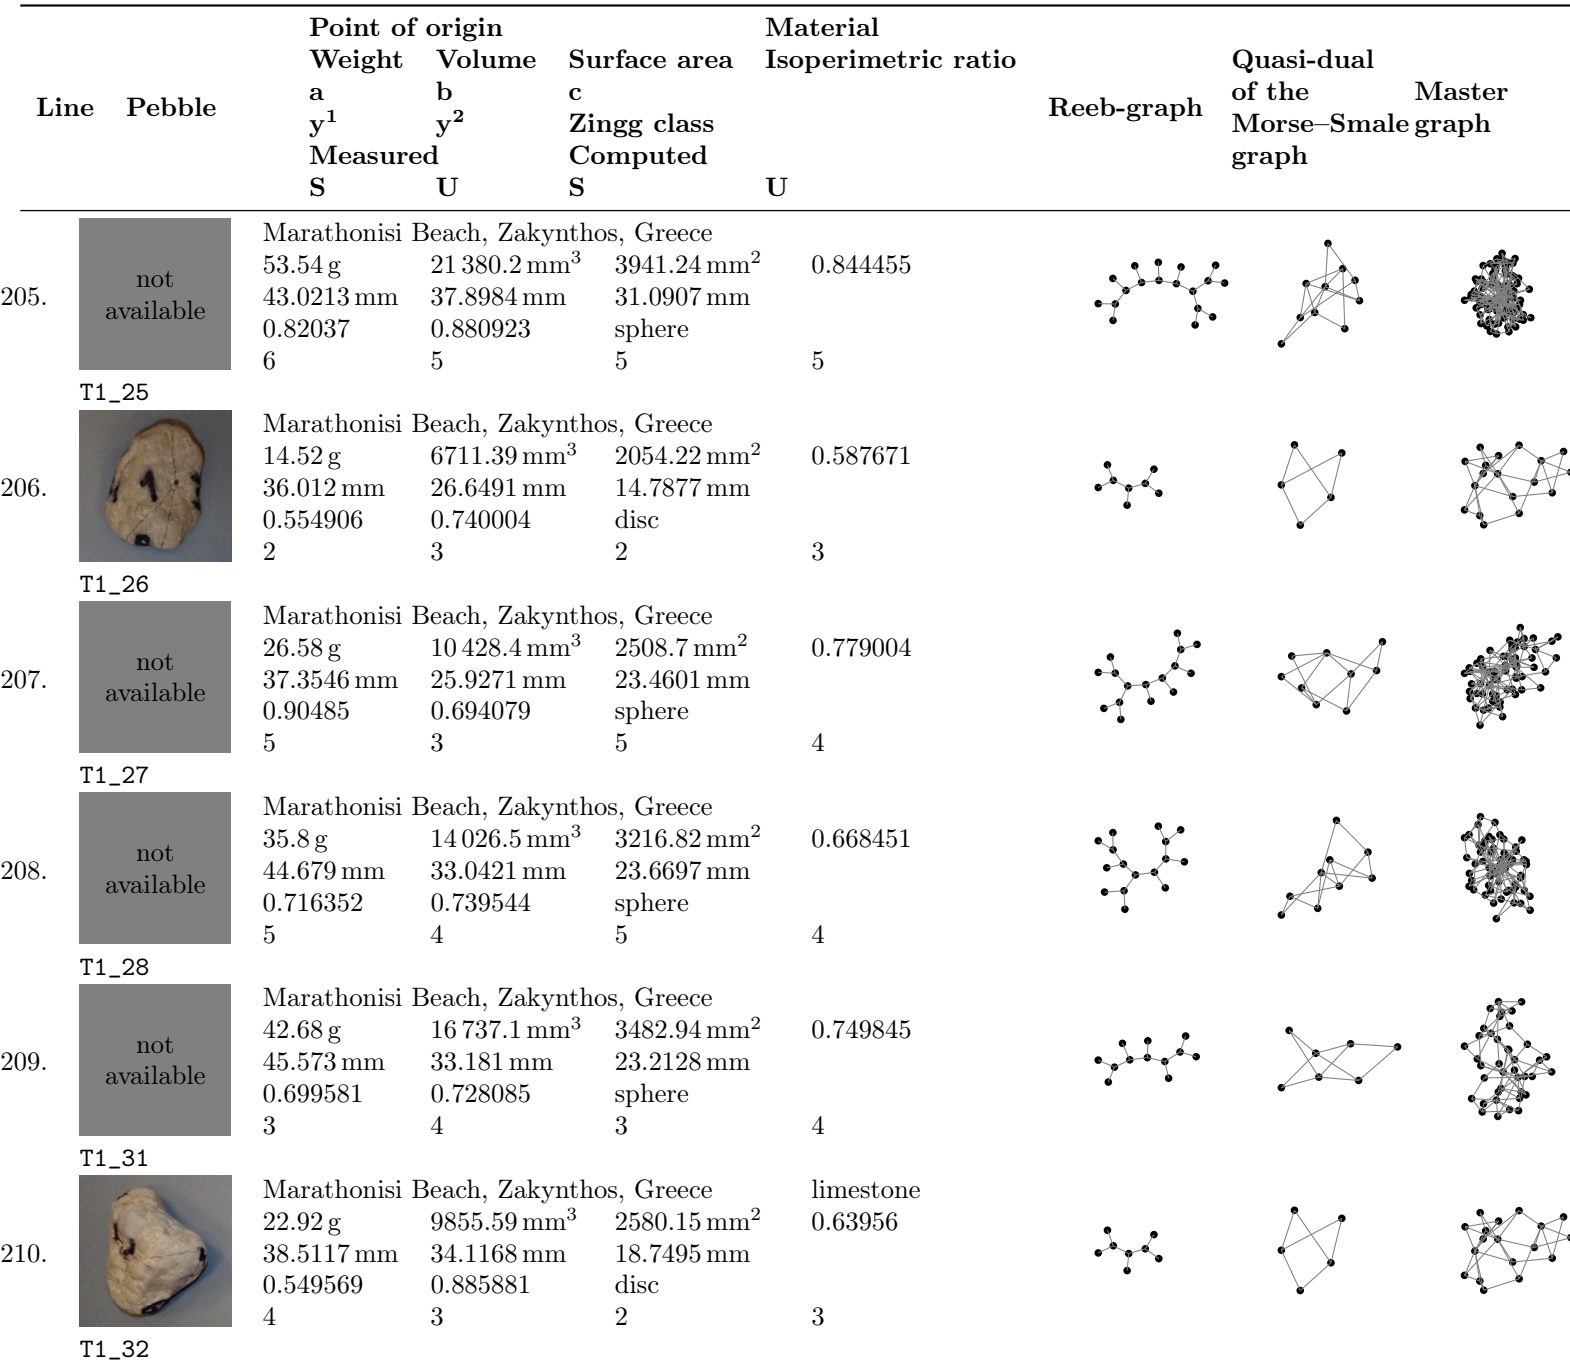   |
|      | T1_27                                                                               |                                                                                |                                                         |                                                      |                                      |                                                                                       |                                                                                       |                                                                                       |
| 208. | 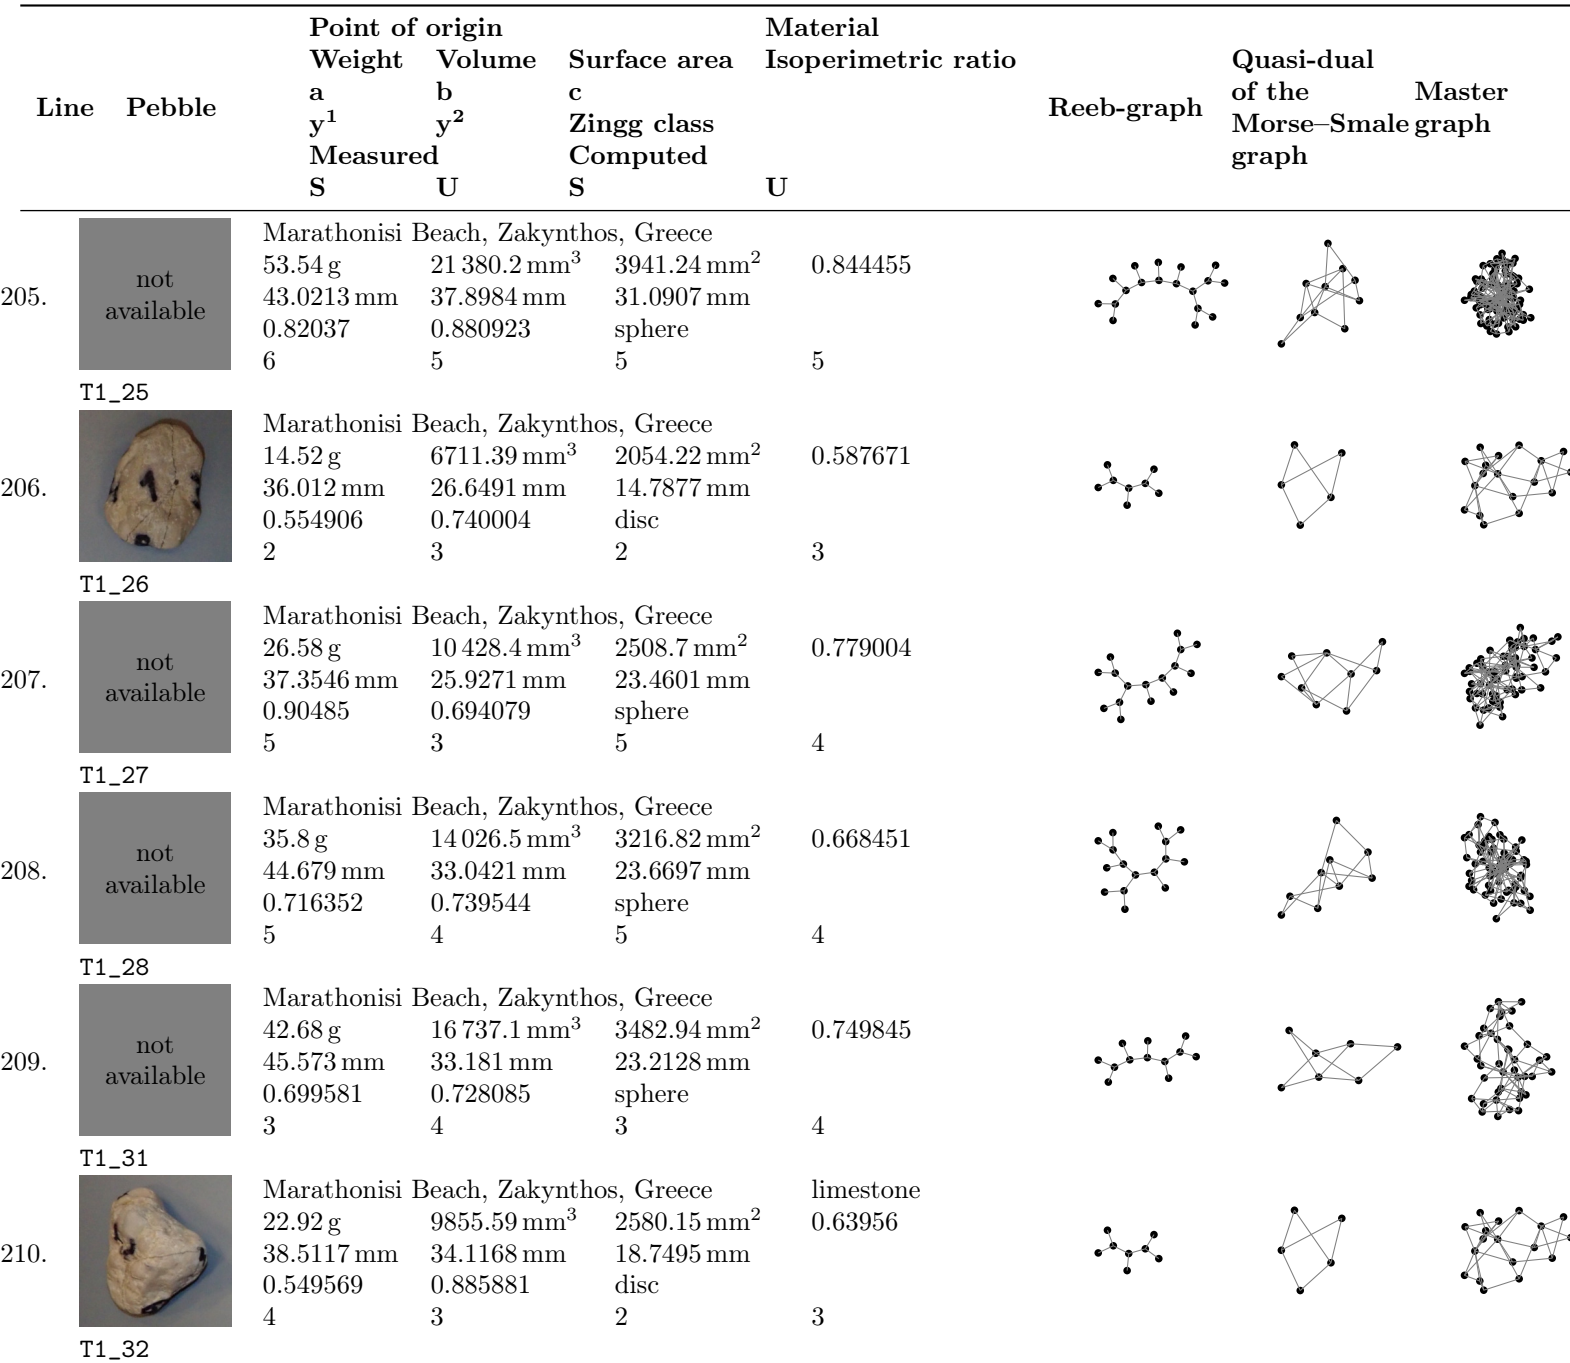  | Marathonisi Beach, Zakynthos, Greece<br>35.8 g<br>44.679 mm<br>0.716352<br>5   | 14 026.5 mm <sup>3</sup><br>33.0421 mm<br>0.739544<br>4 | 3216.82 mm <sup>2</sup><br>23.6697 mm<br>sphere<br>5 | 0.668451                             | 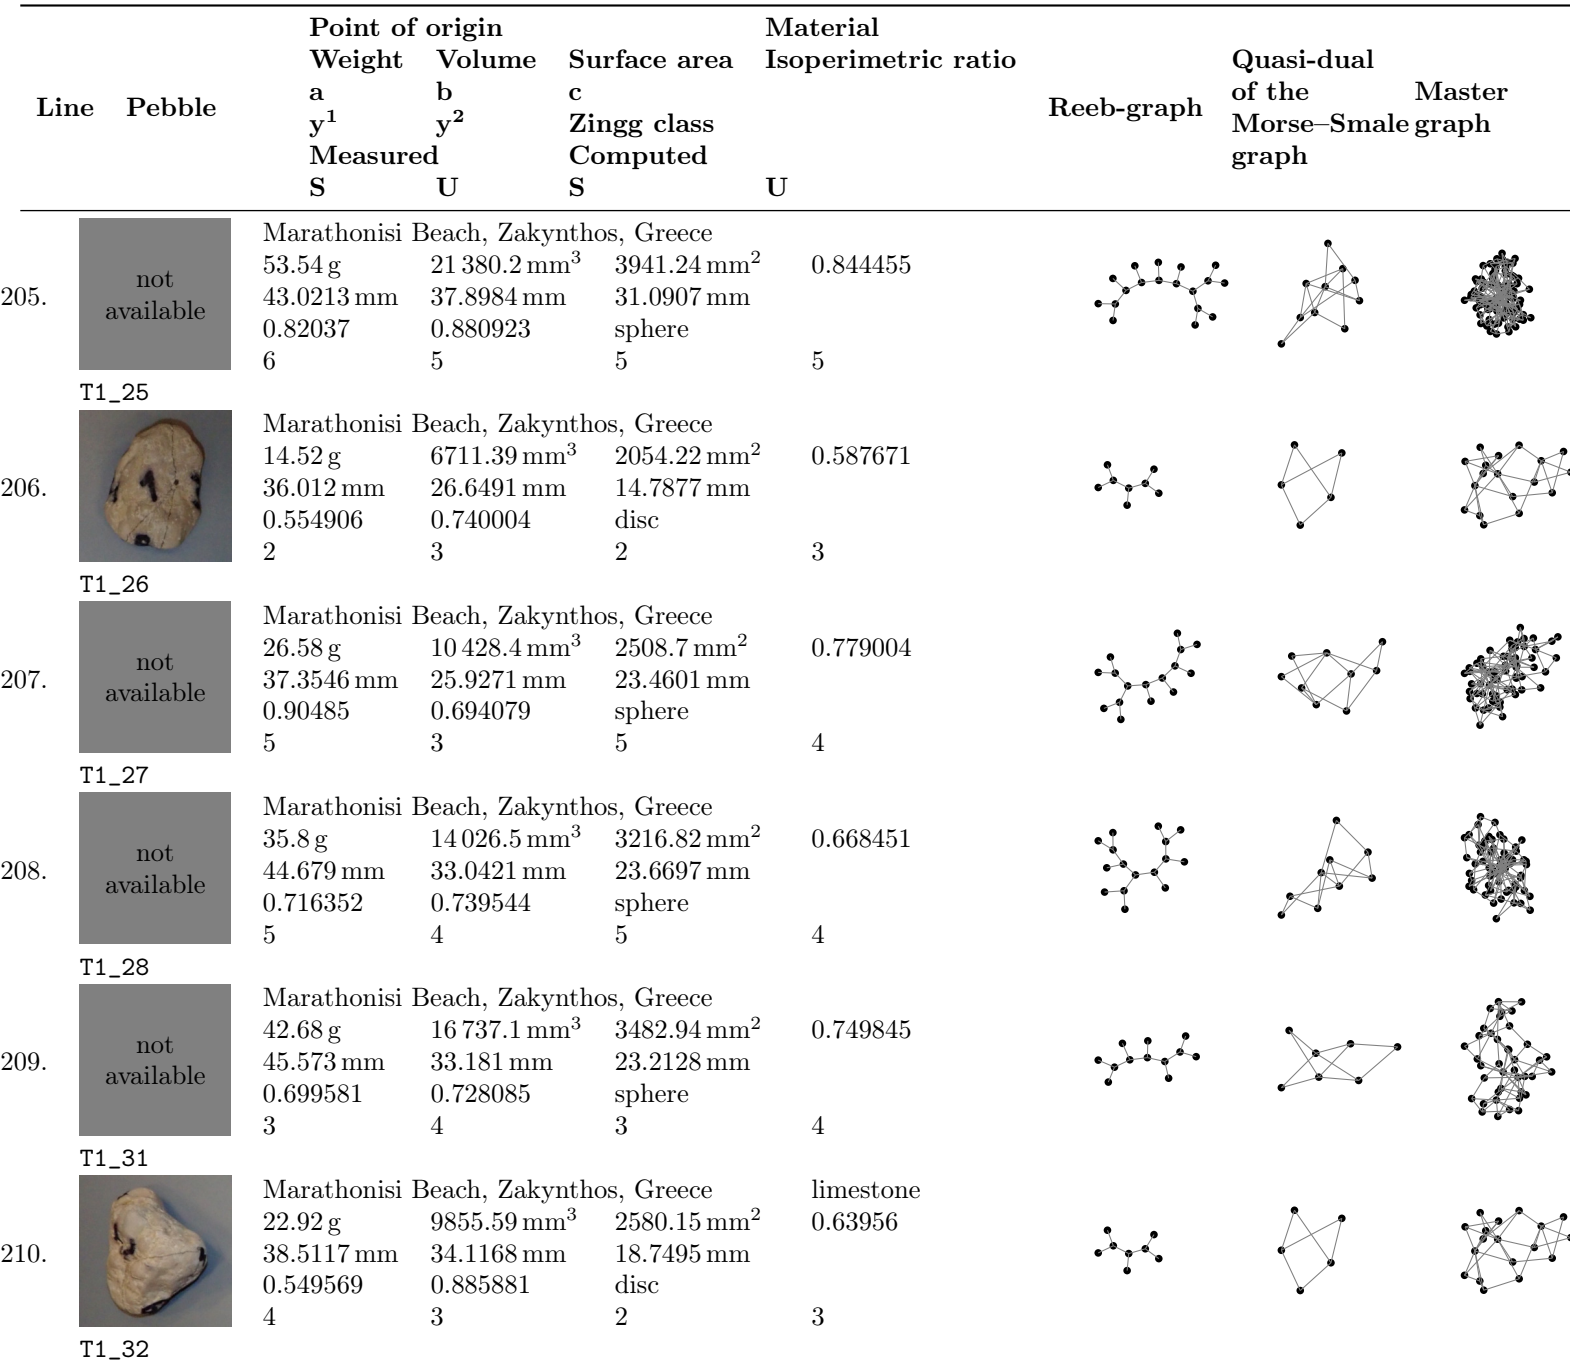  | 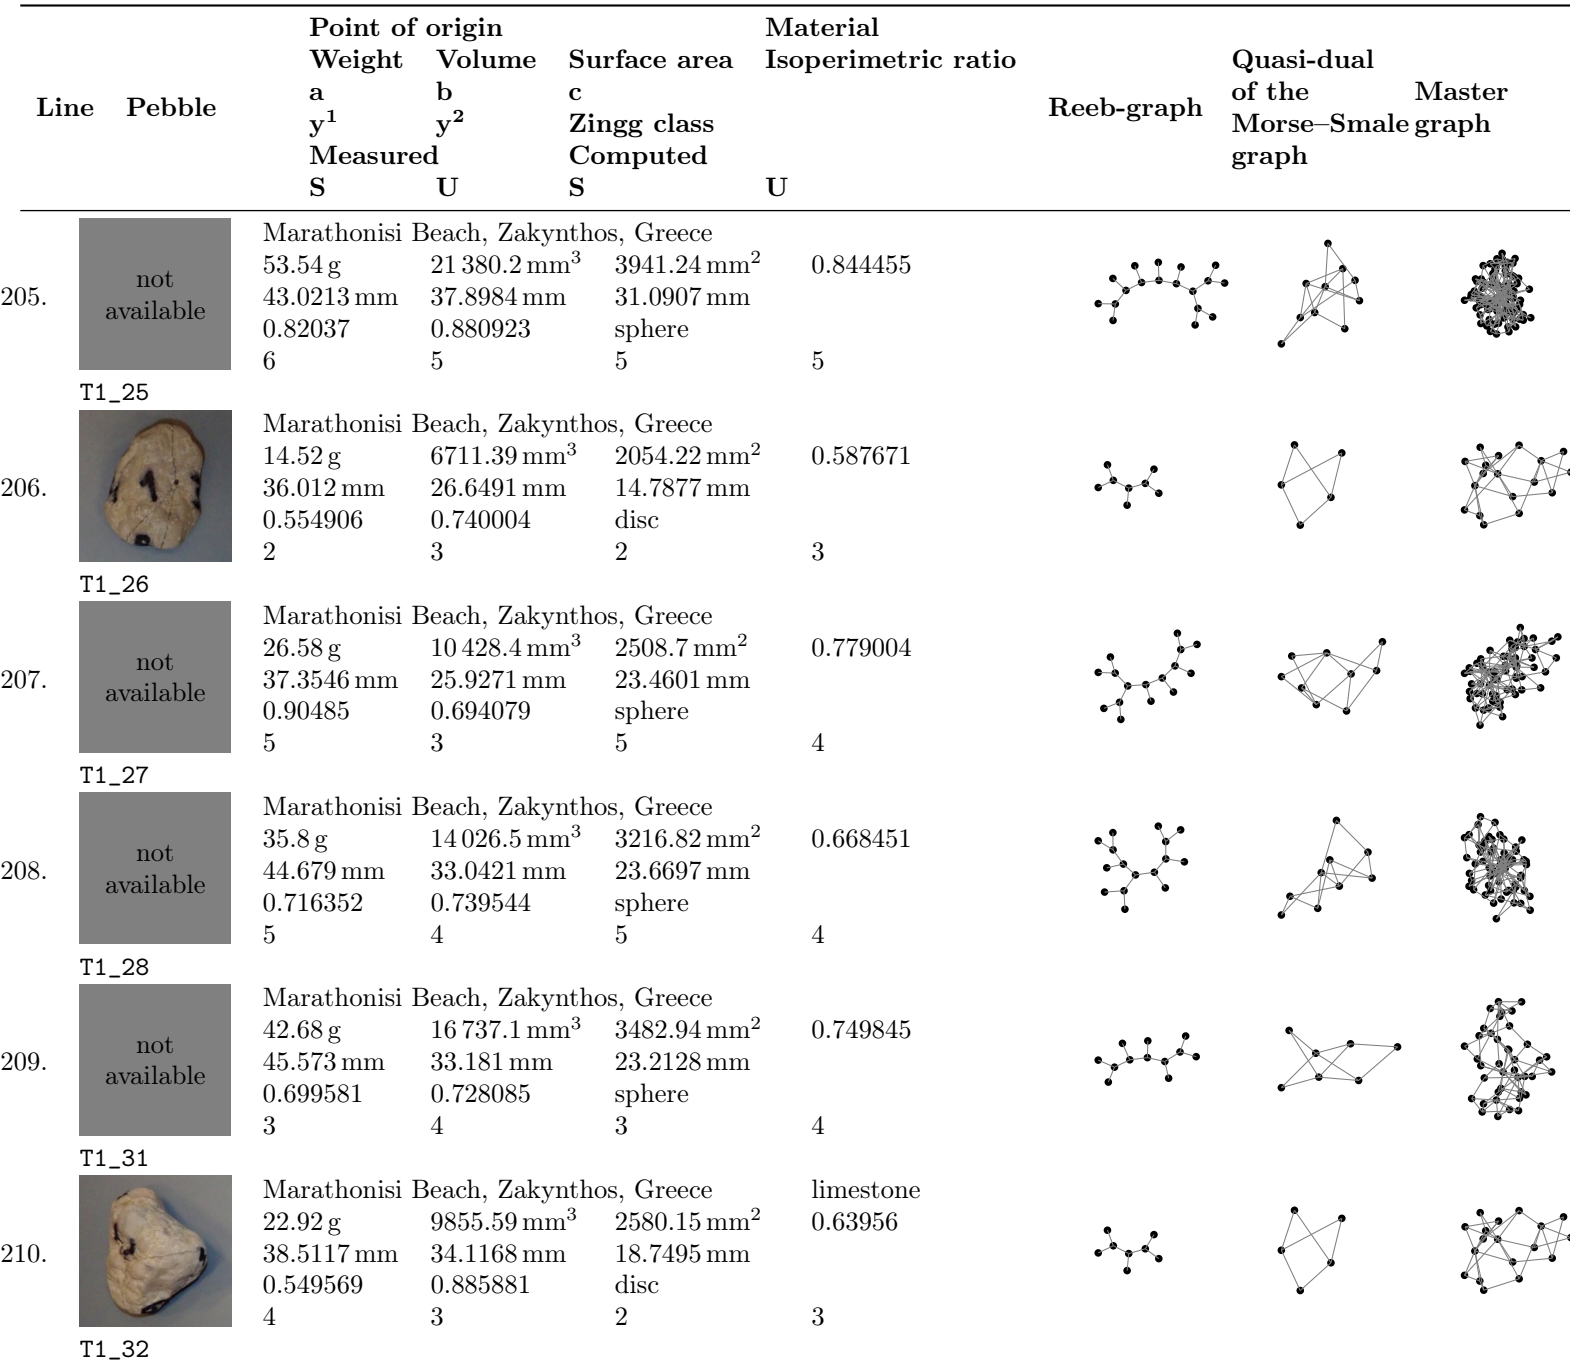  | 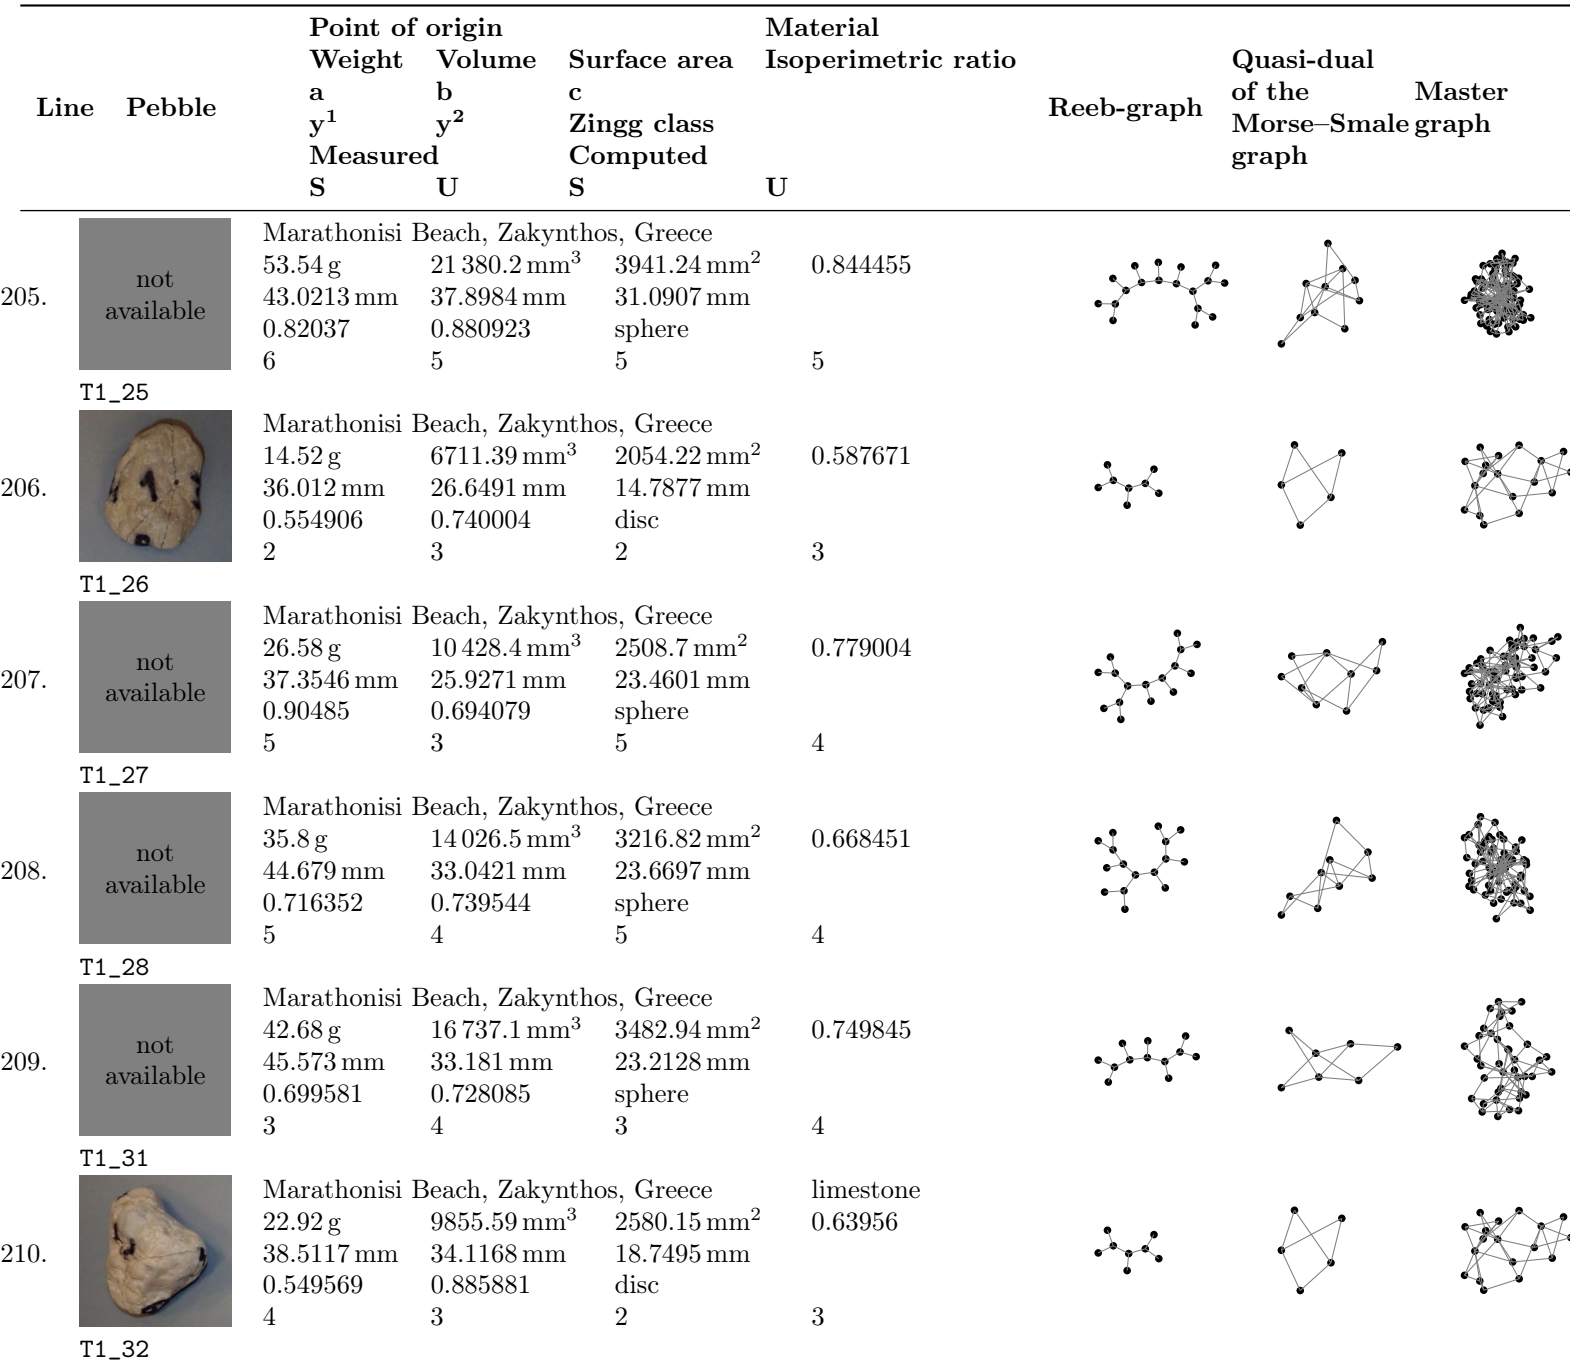  |
|      | T1_28                                                                               |                                                                                |                                                         |                                                      |                                      |                                                                                       |                                                                                       |                                                                                       |
| 209. | 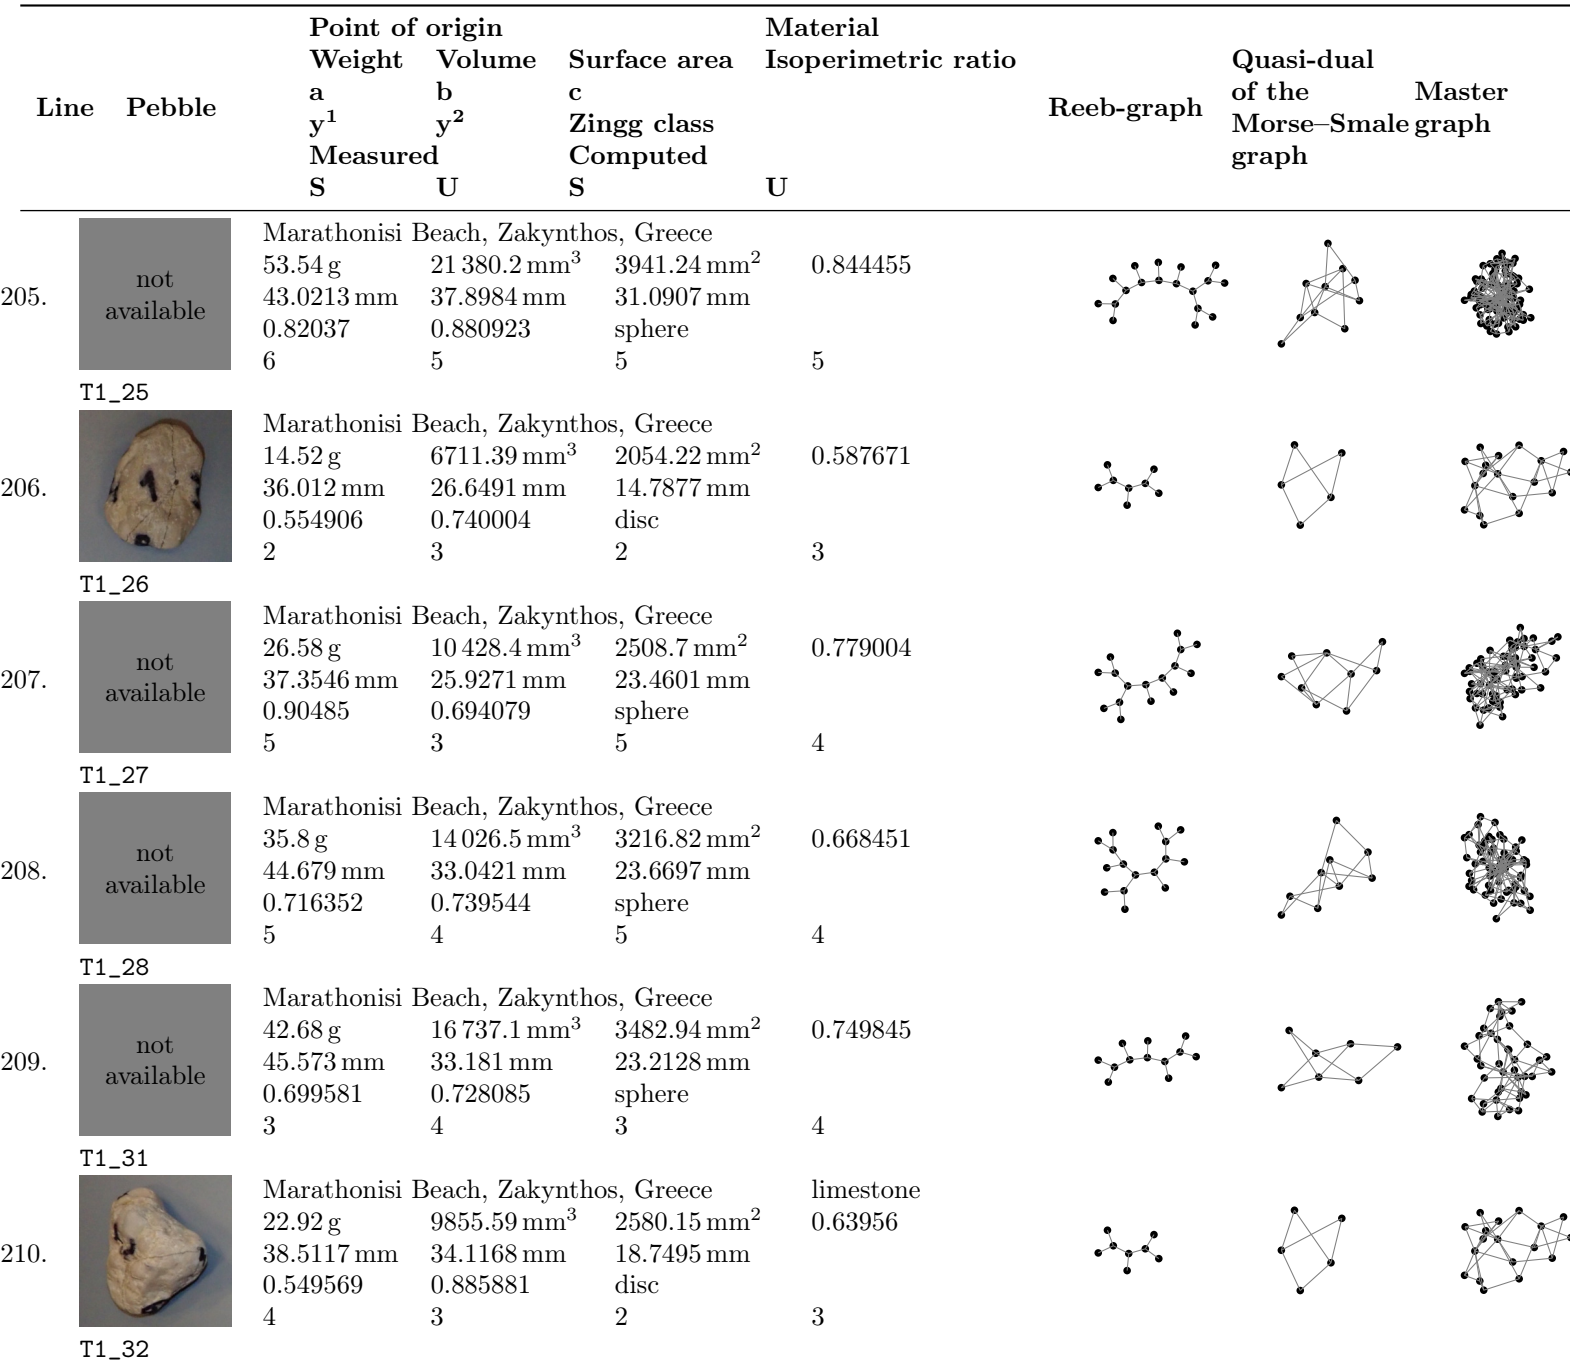 | Marathonisi Beach, Zakynthos, Greece<br>42.68 g<br>45.573 mm<br>0.699581<br>3  | 16 737.1 mm <sup>3</sup><br>33.181 mm<br>0.728085<br>4  | 3482.94 mm <sup>2</sup><br>23.2128 mm<br>sphere<br>3 | 0.749845                             | 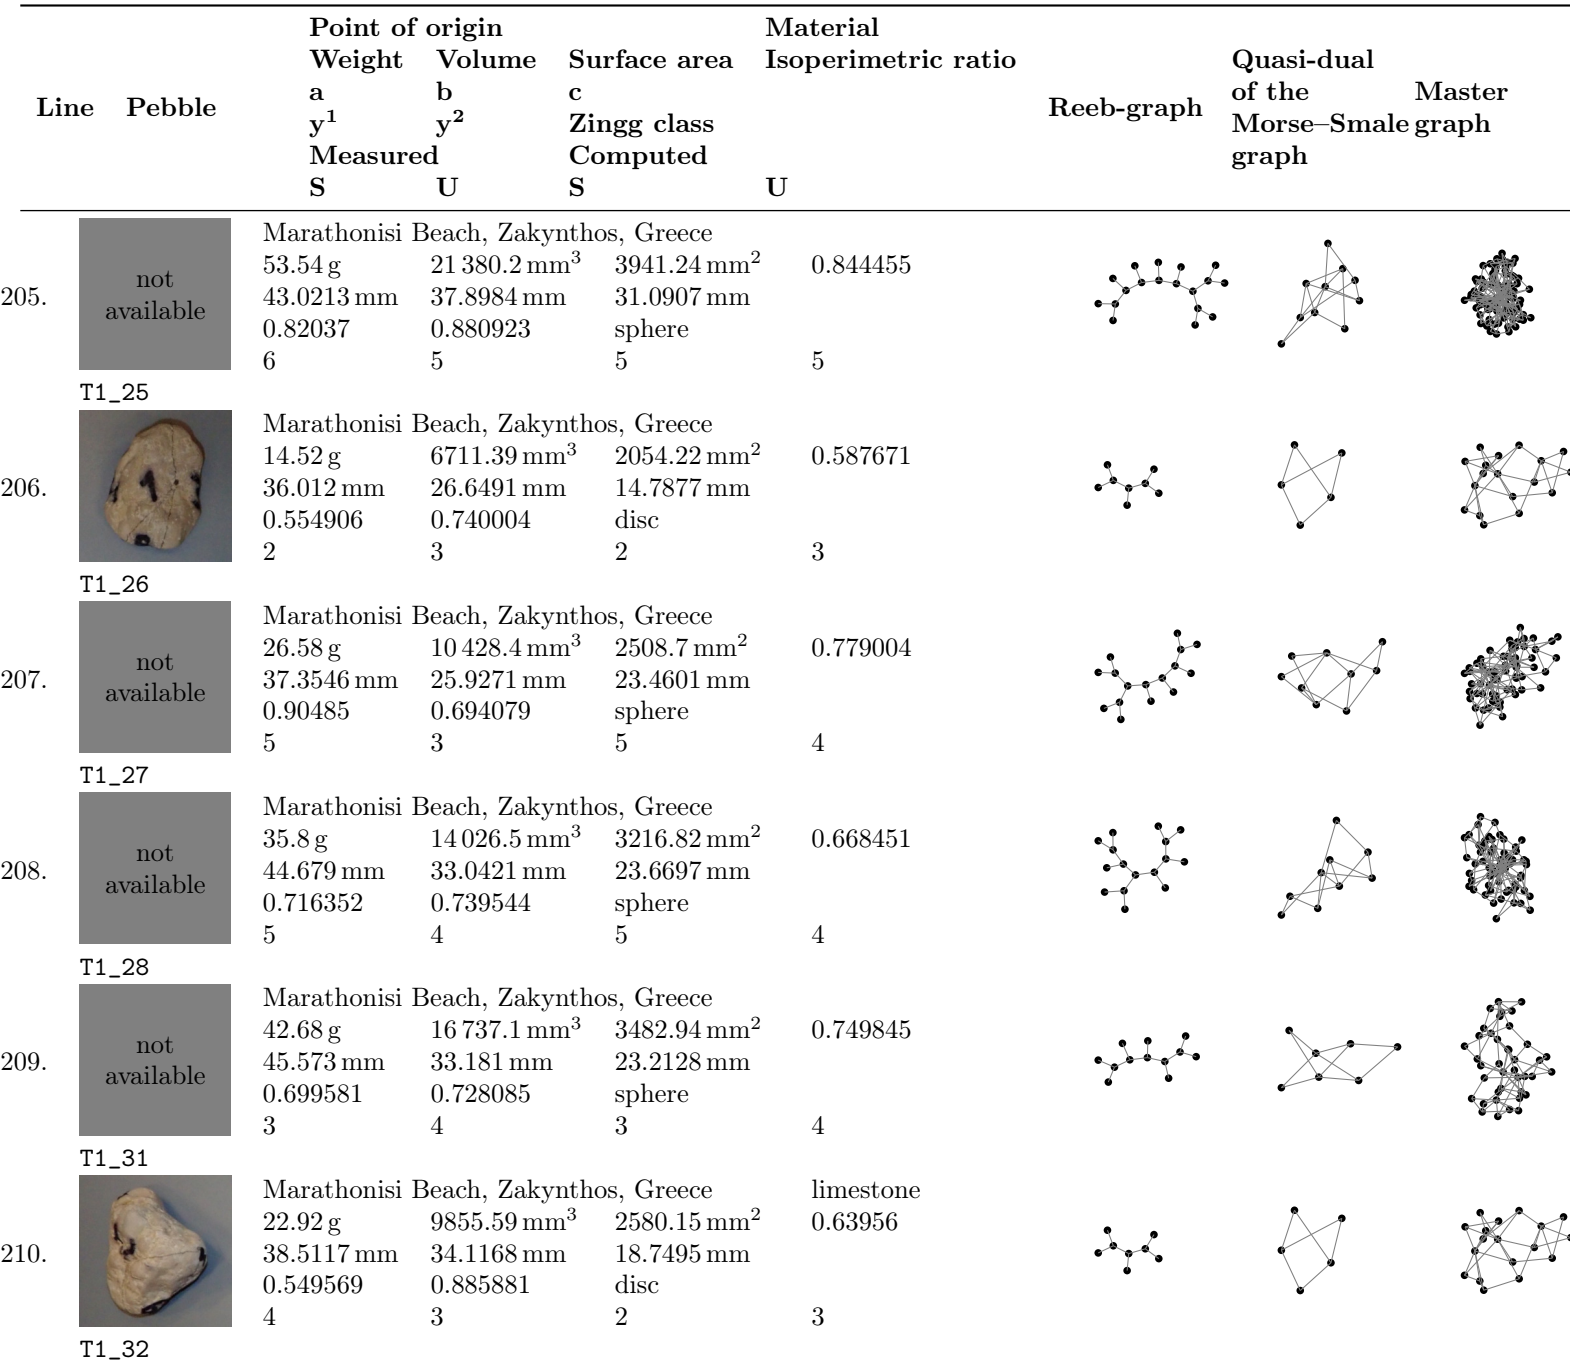 | 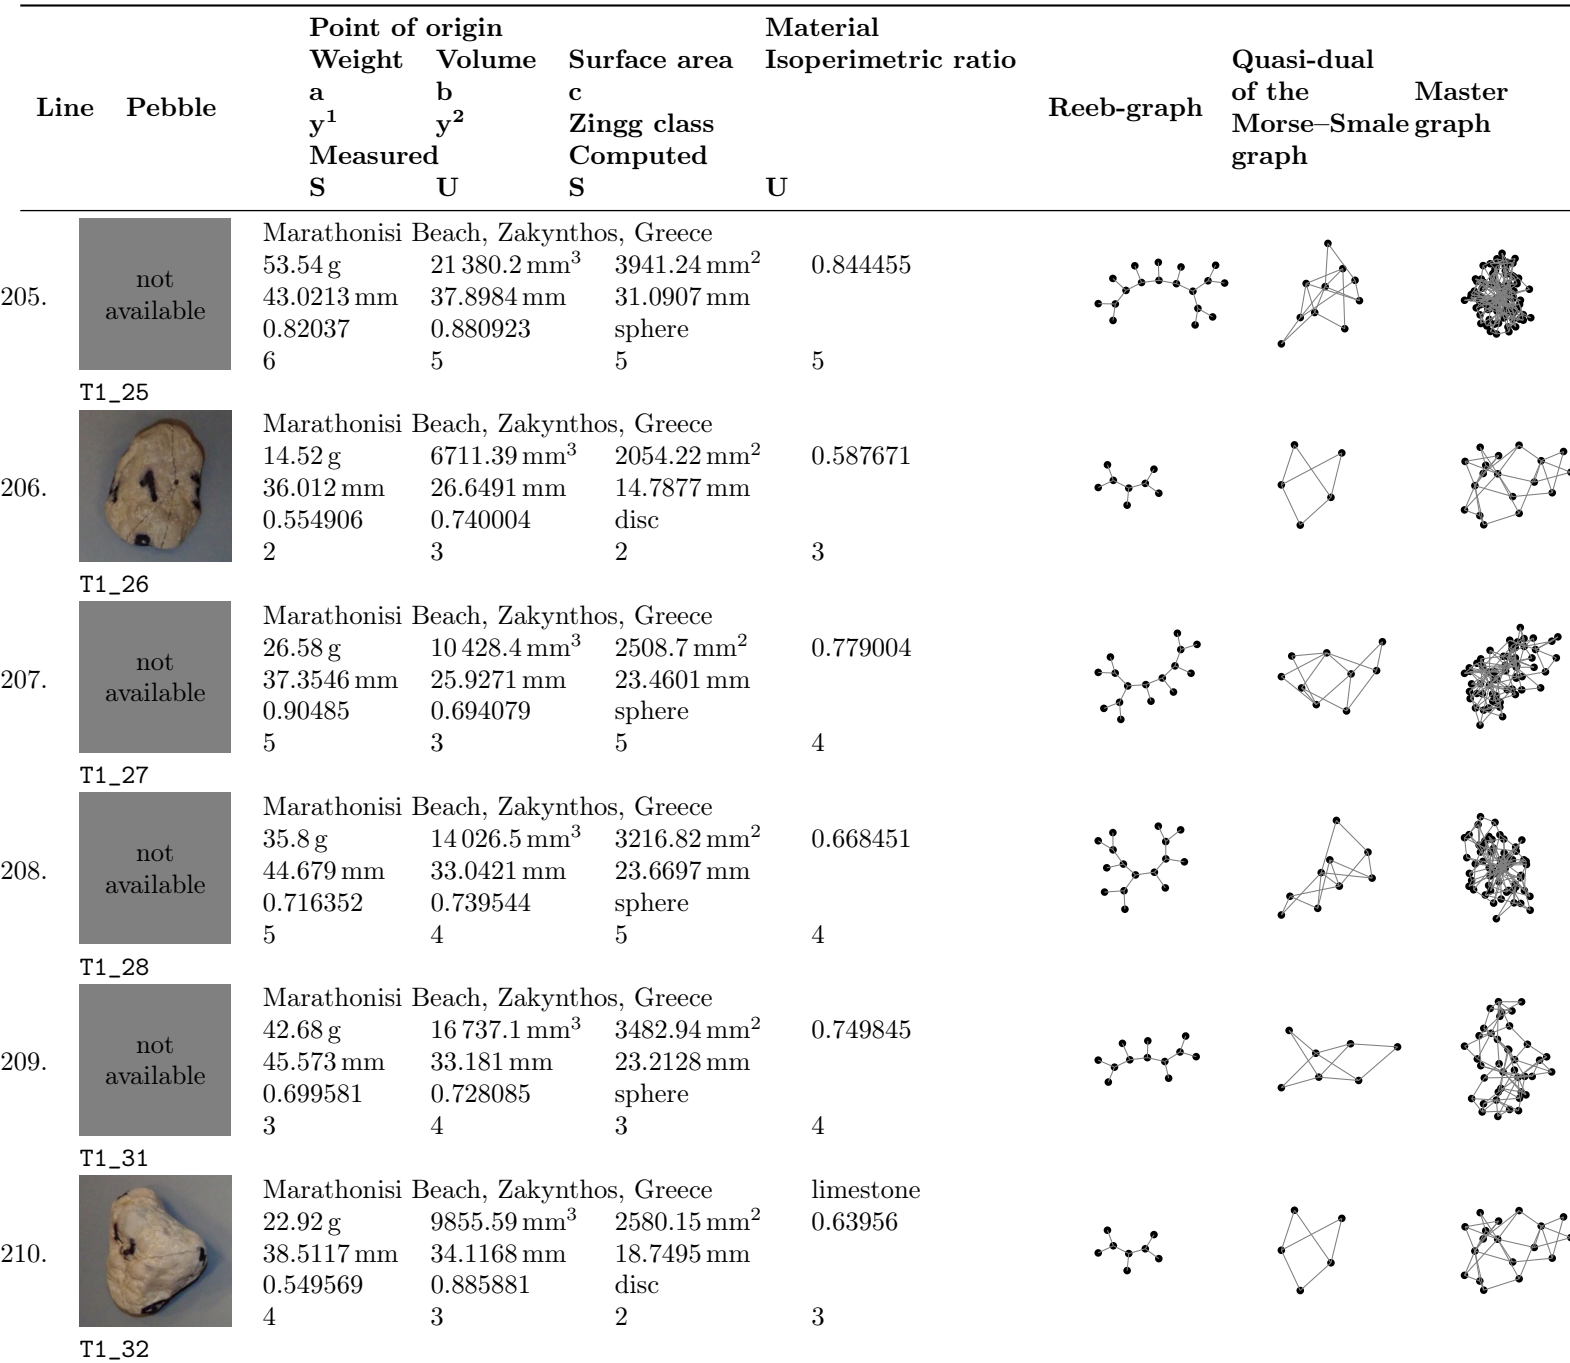 | 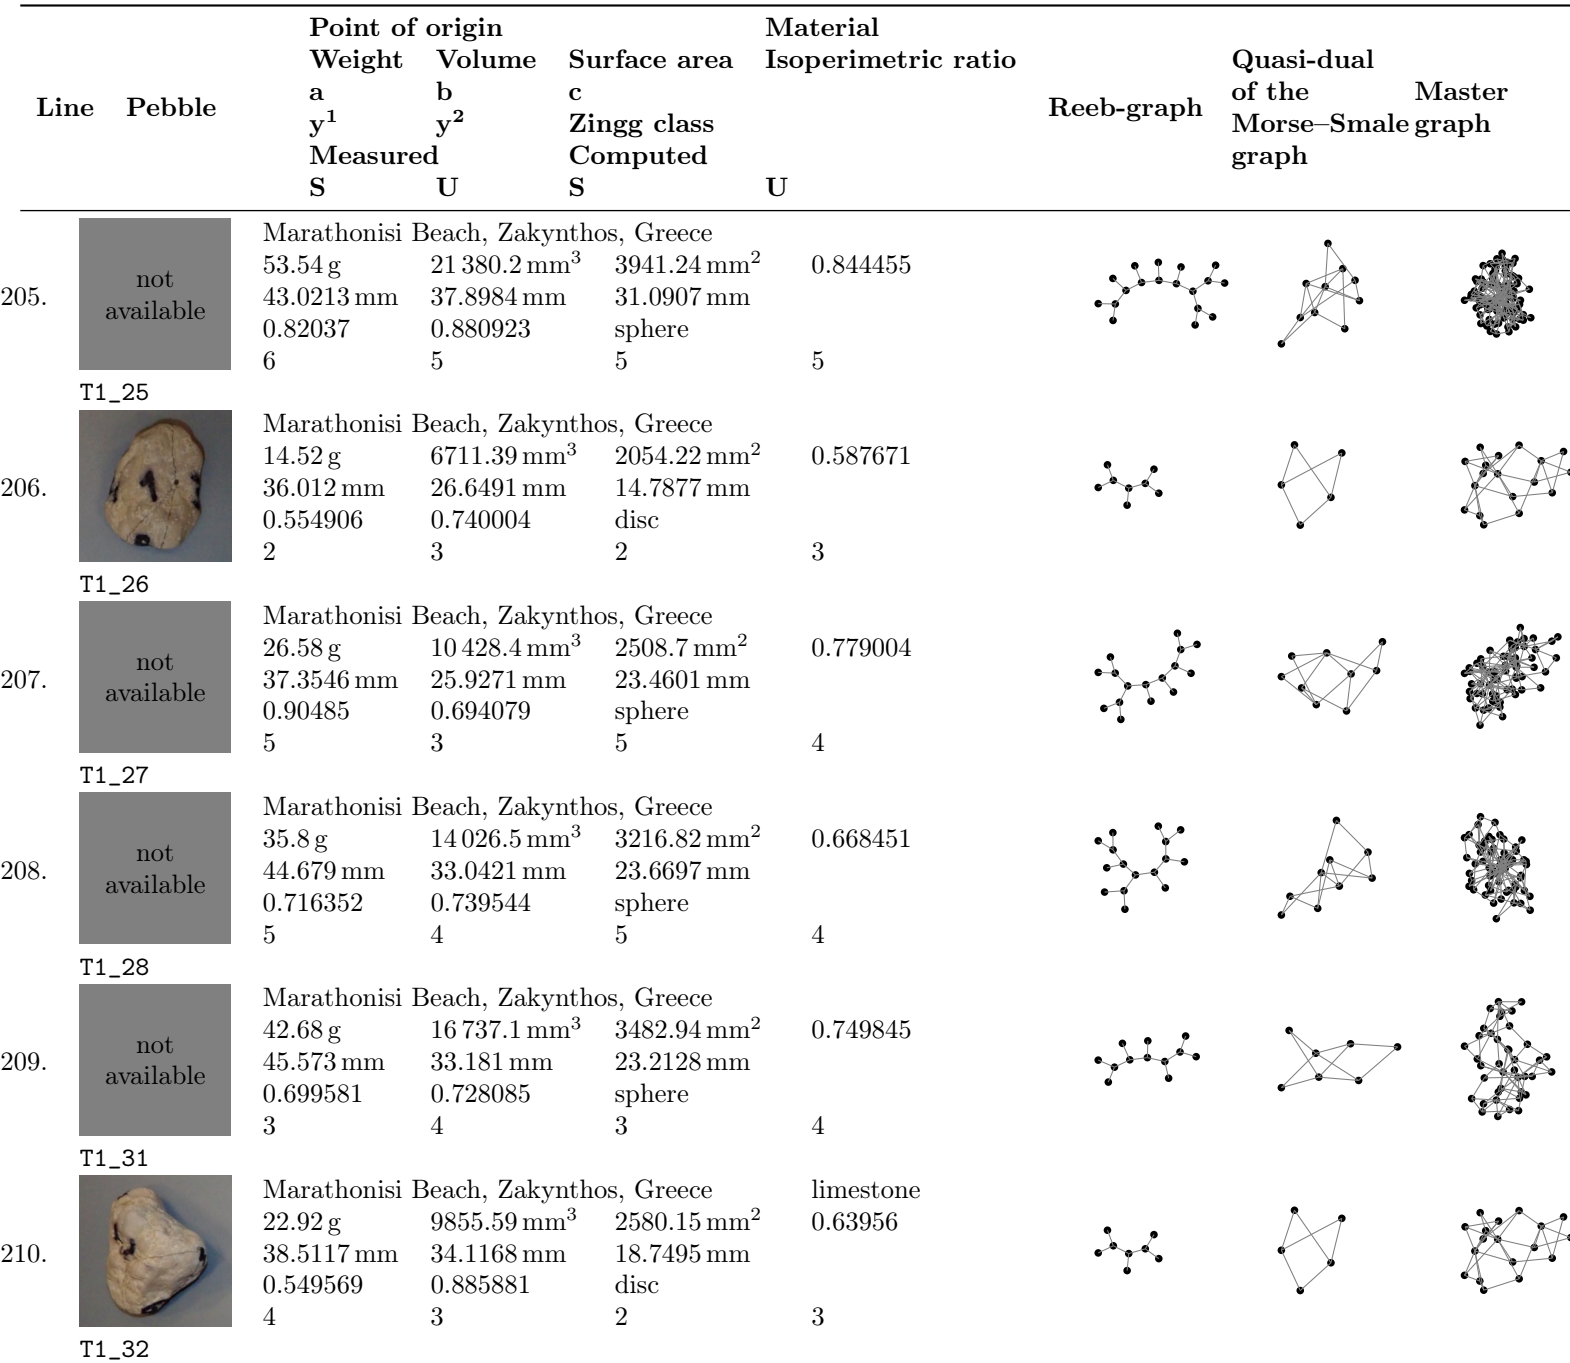 |
|      | T1_31                                                                               |                                                                                |                                                         |                                                      |                                      |                                                                                       |                                                                                       |                                                                                       |
| 210. | 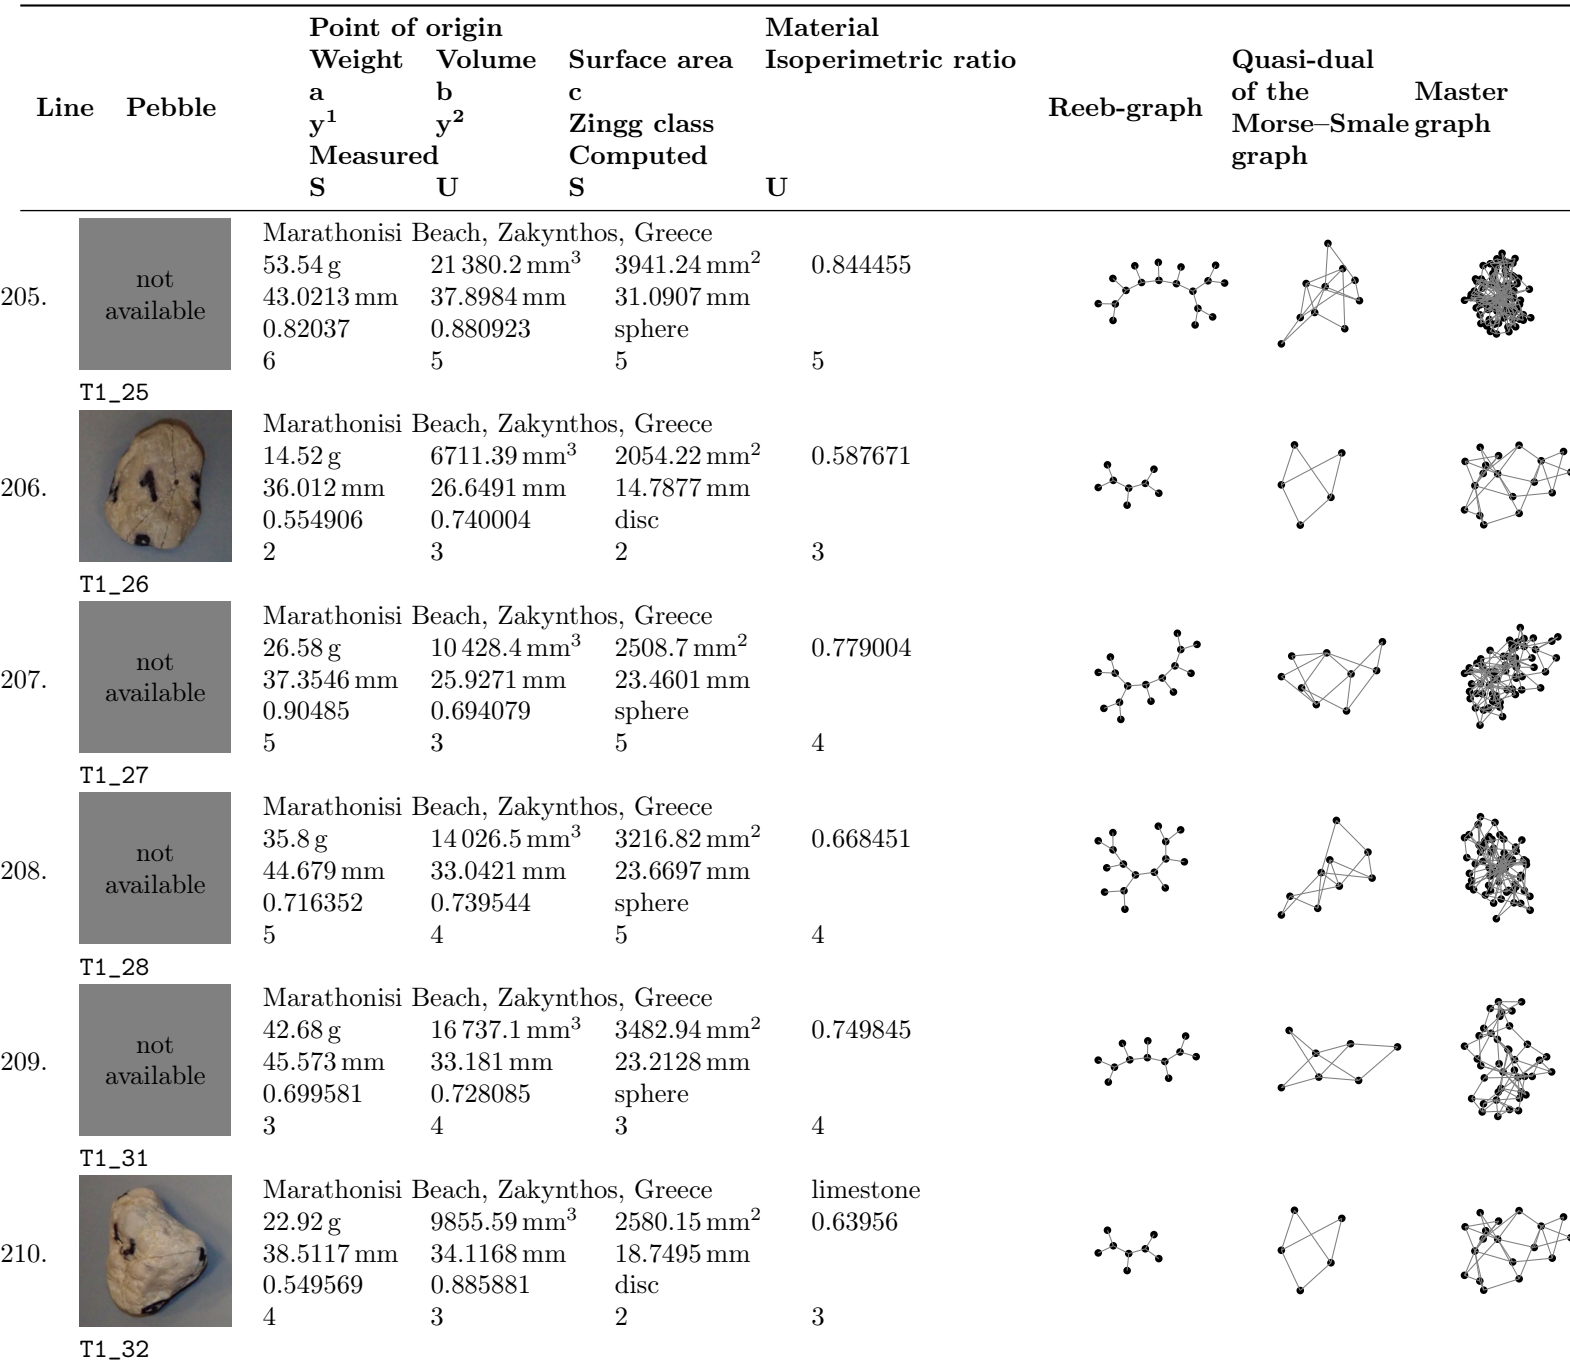 | Marathonisi Beach, Zakynthos, Greece<br>22.92 g<br>38.5117 mm<br>0.549569<br>4 | 9855.59 mm <sup>3</sup><br>34.1168 mm<br>0.885881<br>3  | 2580.15 mm <sup>2</sup><br>18.7495 mm<br>disc<br>2   | limestone<br>0.63956<br>3            | 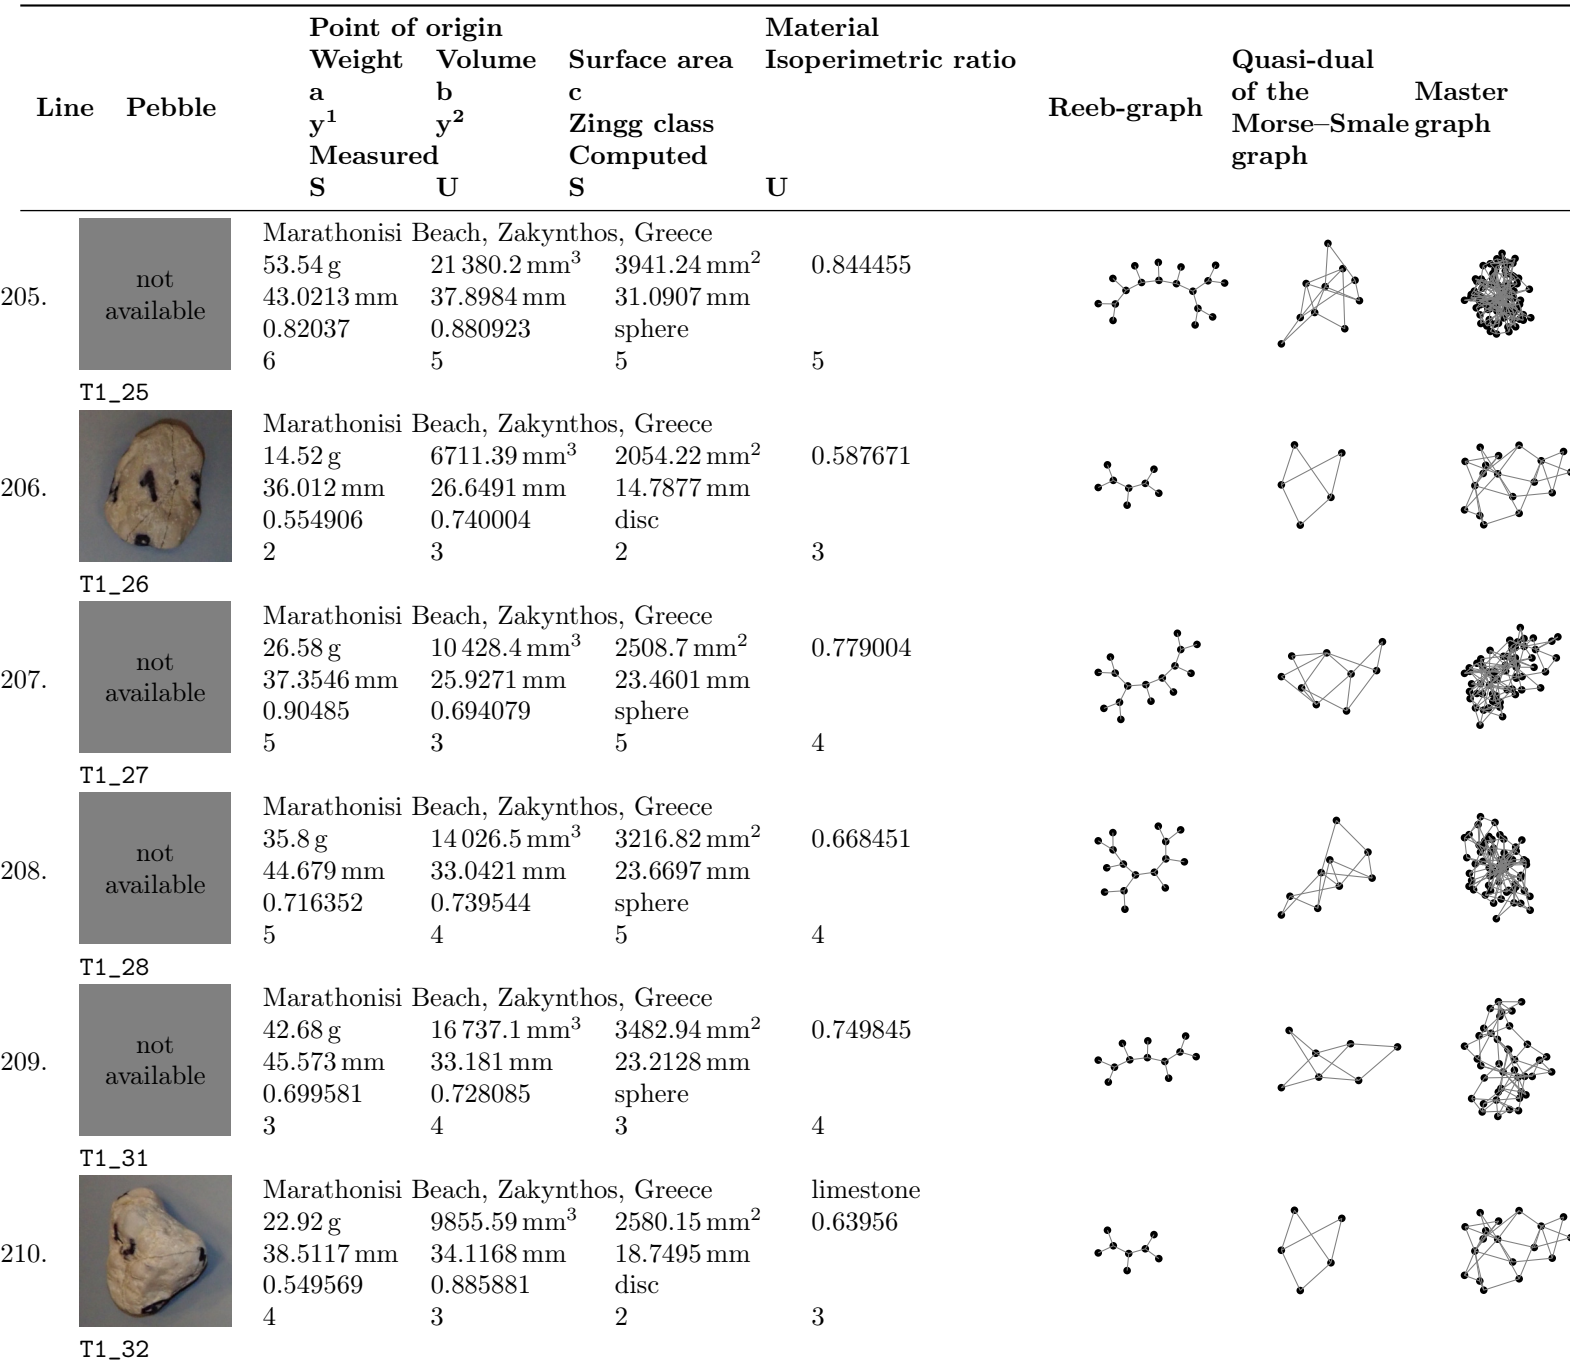 | 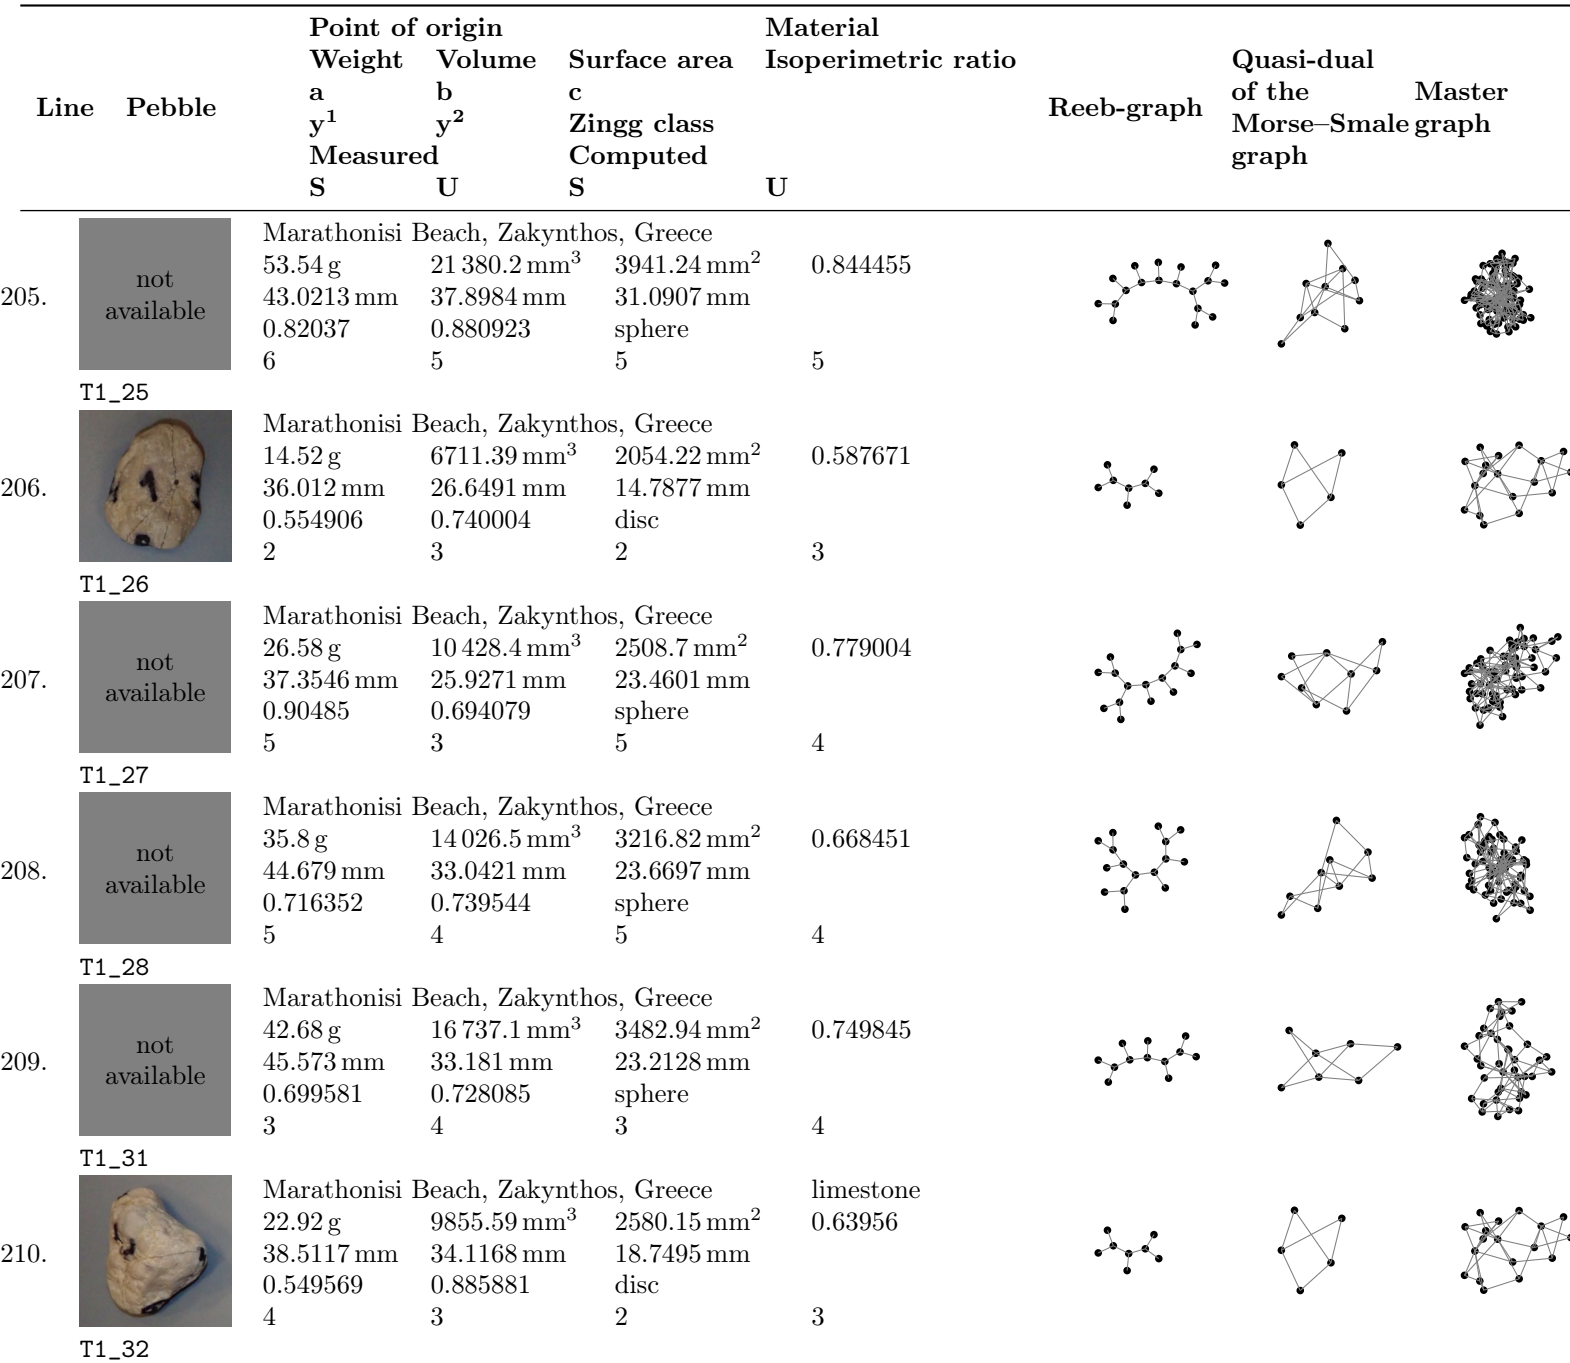 | 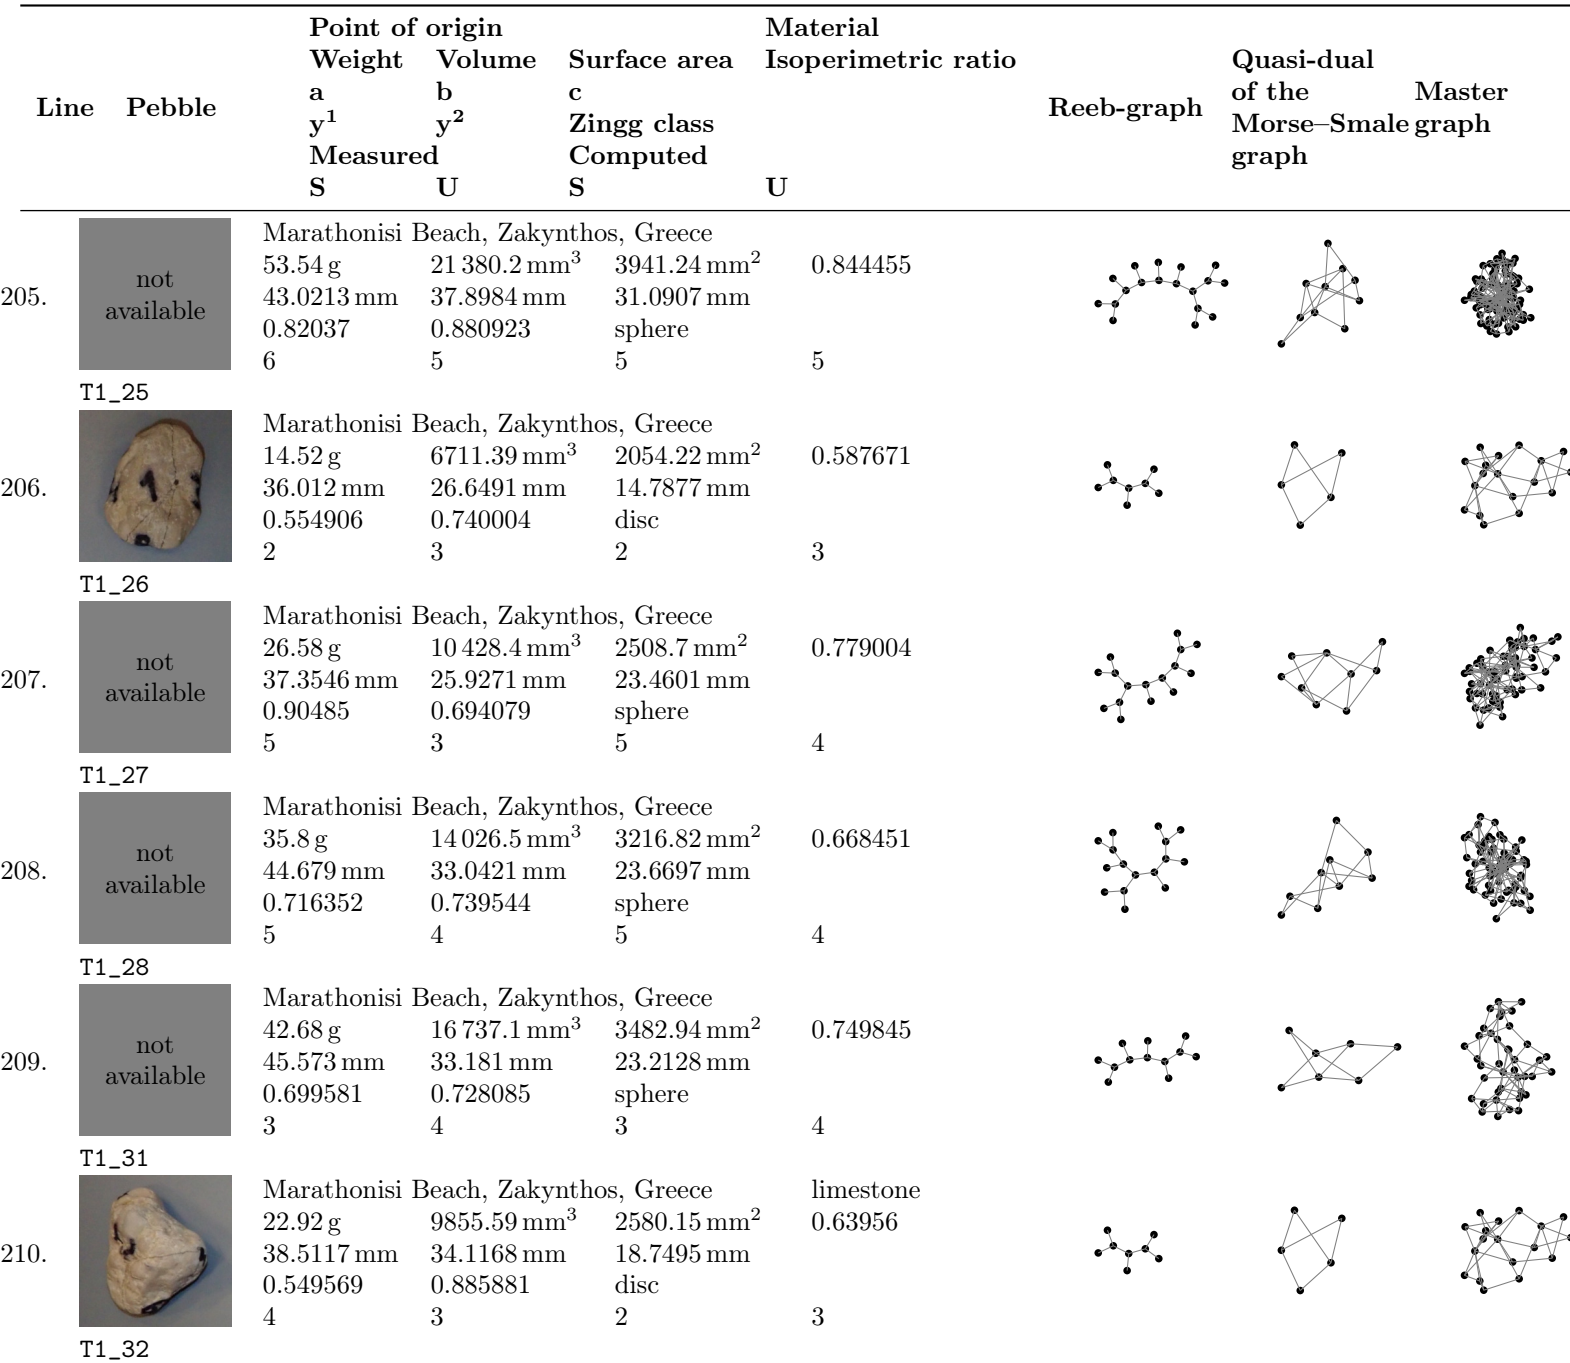 |
|      | T1_32                                                                               |                                                                                |                                                         |                                                      |                                      |                                                                                       |                                                                                       |                                                                                       |

| Line | Pebble                                                                              | Point of origin                      |                          | Surface area            | Material            | Reeb-graph                                                                            | Quasi-dual<br>of the<br>Morse–Smale<br>graph                                          | Master<br>graph                                                                       |
|------|-------------------------------------------------------------------------------------|--------------------------------------|--------------------------|-------------------------|---------------------|---------------------------------------------------------------------------------------|---------------------------------------------------------------------------------------|---------------------------------------------------------------------------------------|
|      |                                                                                     | Weight                               | Volume                   |                         |                     |                                                                                       |                                                                                       |                                                                                       |
|      |                                                                                     | a                                    | b                        |                         |                     |                                                                                       |                                                                                       |                                                                                       |
|      |                                                                                     | y <sup>1</sup>                       | y <sup>2</sup>           |                         |                     |                                                                                       |                                                                                       |                                                                                       |
|      |                                                                                     | Measured                             |                          | Zingg class             | Isoperimetric ratio |                                                                                       |                                                                                       |                                                                                       |
|      |                                                                                     | S                                    | U                        | Computed                | U                   |                                                                                       |                                                                                       |                                                                                       |
| 211. | 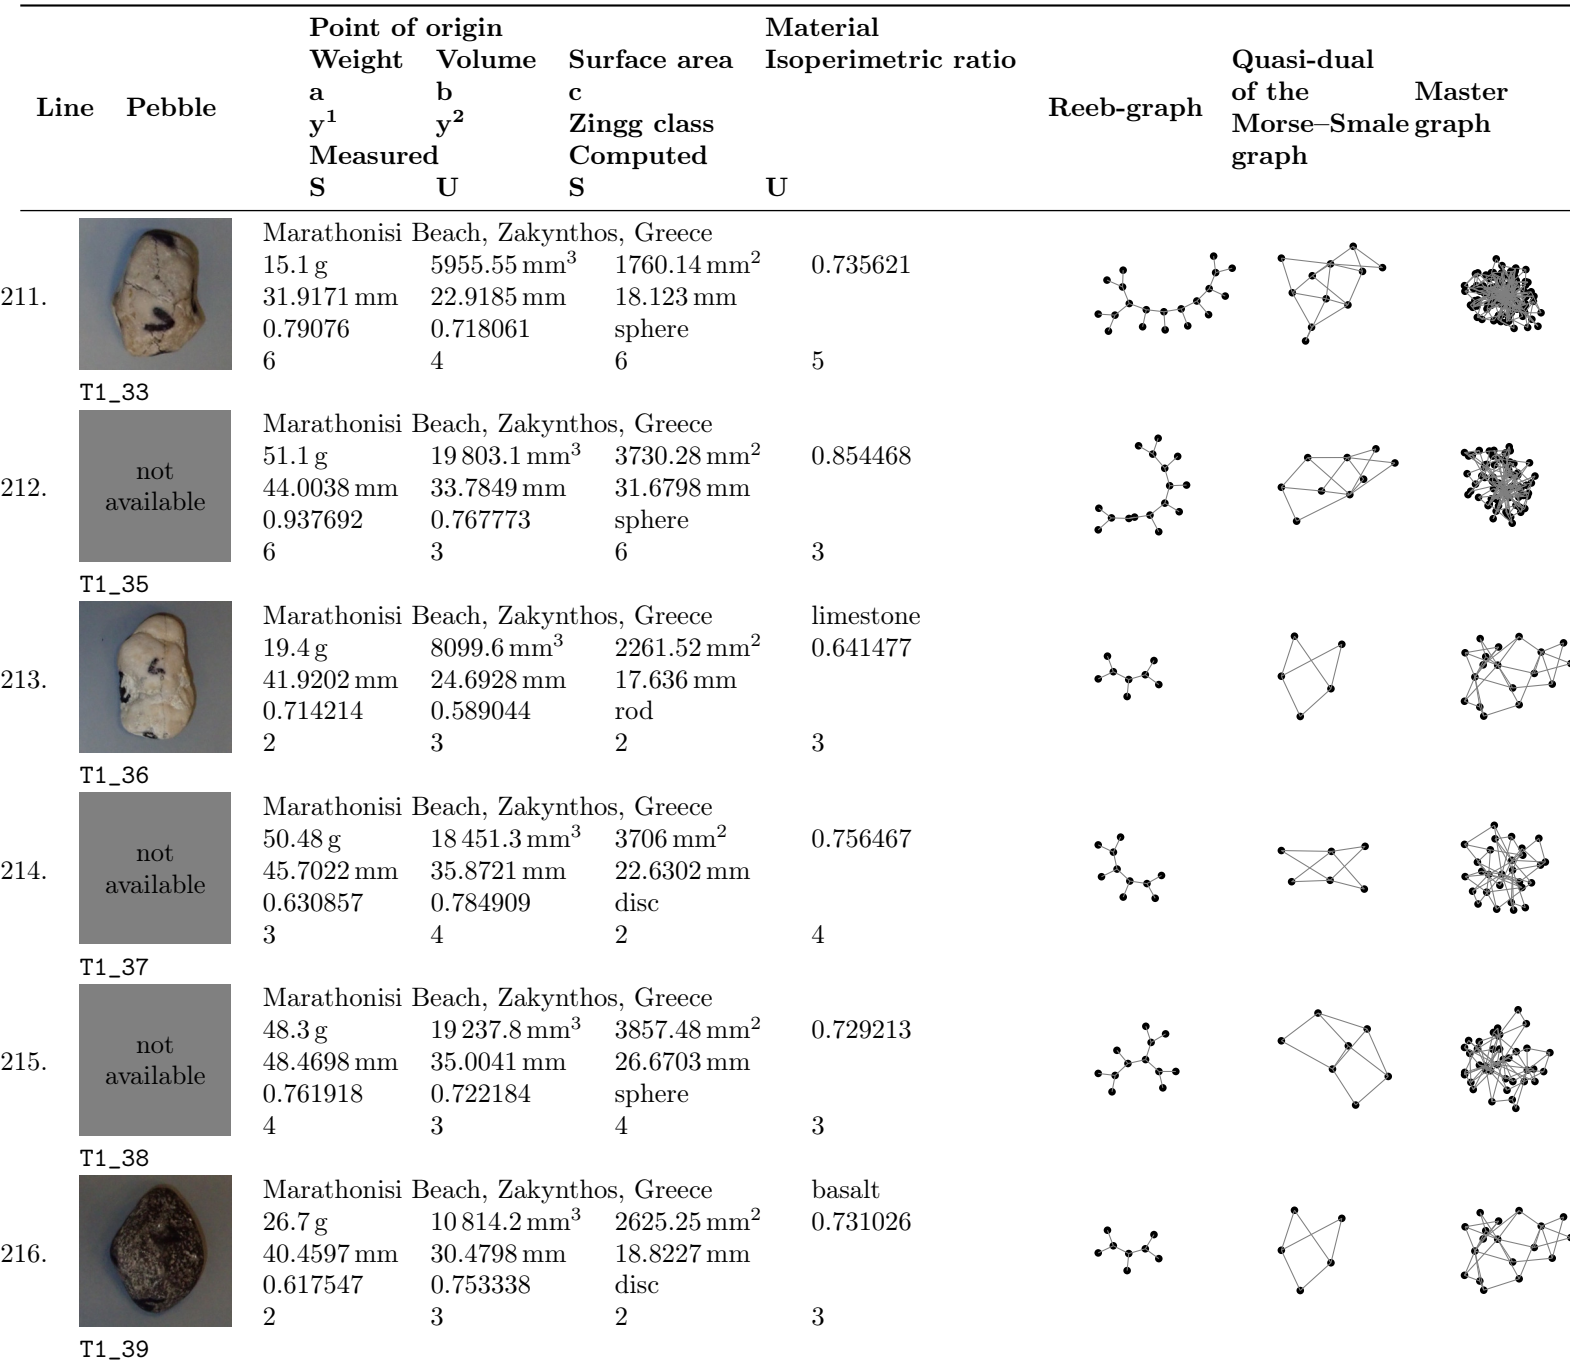   | Marathonisi Beach, Zakynthos, Greece |                          |                         |                     |                                                                                       |                                                                                       |                                                                                       |
|      |                                                                                     | 15.1 g                               | 5955.55 mm <sup>3</sup>  | 1760.14 mm <sup>2</sup> | 0.735621            |                                                                                       |                                                                                       |                                                                                       |
|      |                                                                                     | 31.9171 mm                           | 22.9185 mm               | 18.123 mm               |                     |                                                                                       |                                                                                       |                                                                                       |
|      |                                                                                     | 0.79076                              | 0.718061                 | sphere                  |                     |                                                                                       |                                                                                       |                                                                                       |
|      |                                                                                     | 6                                    | 4                        | 6                       | 5                   | 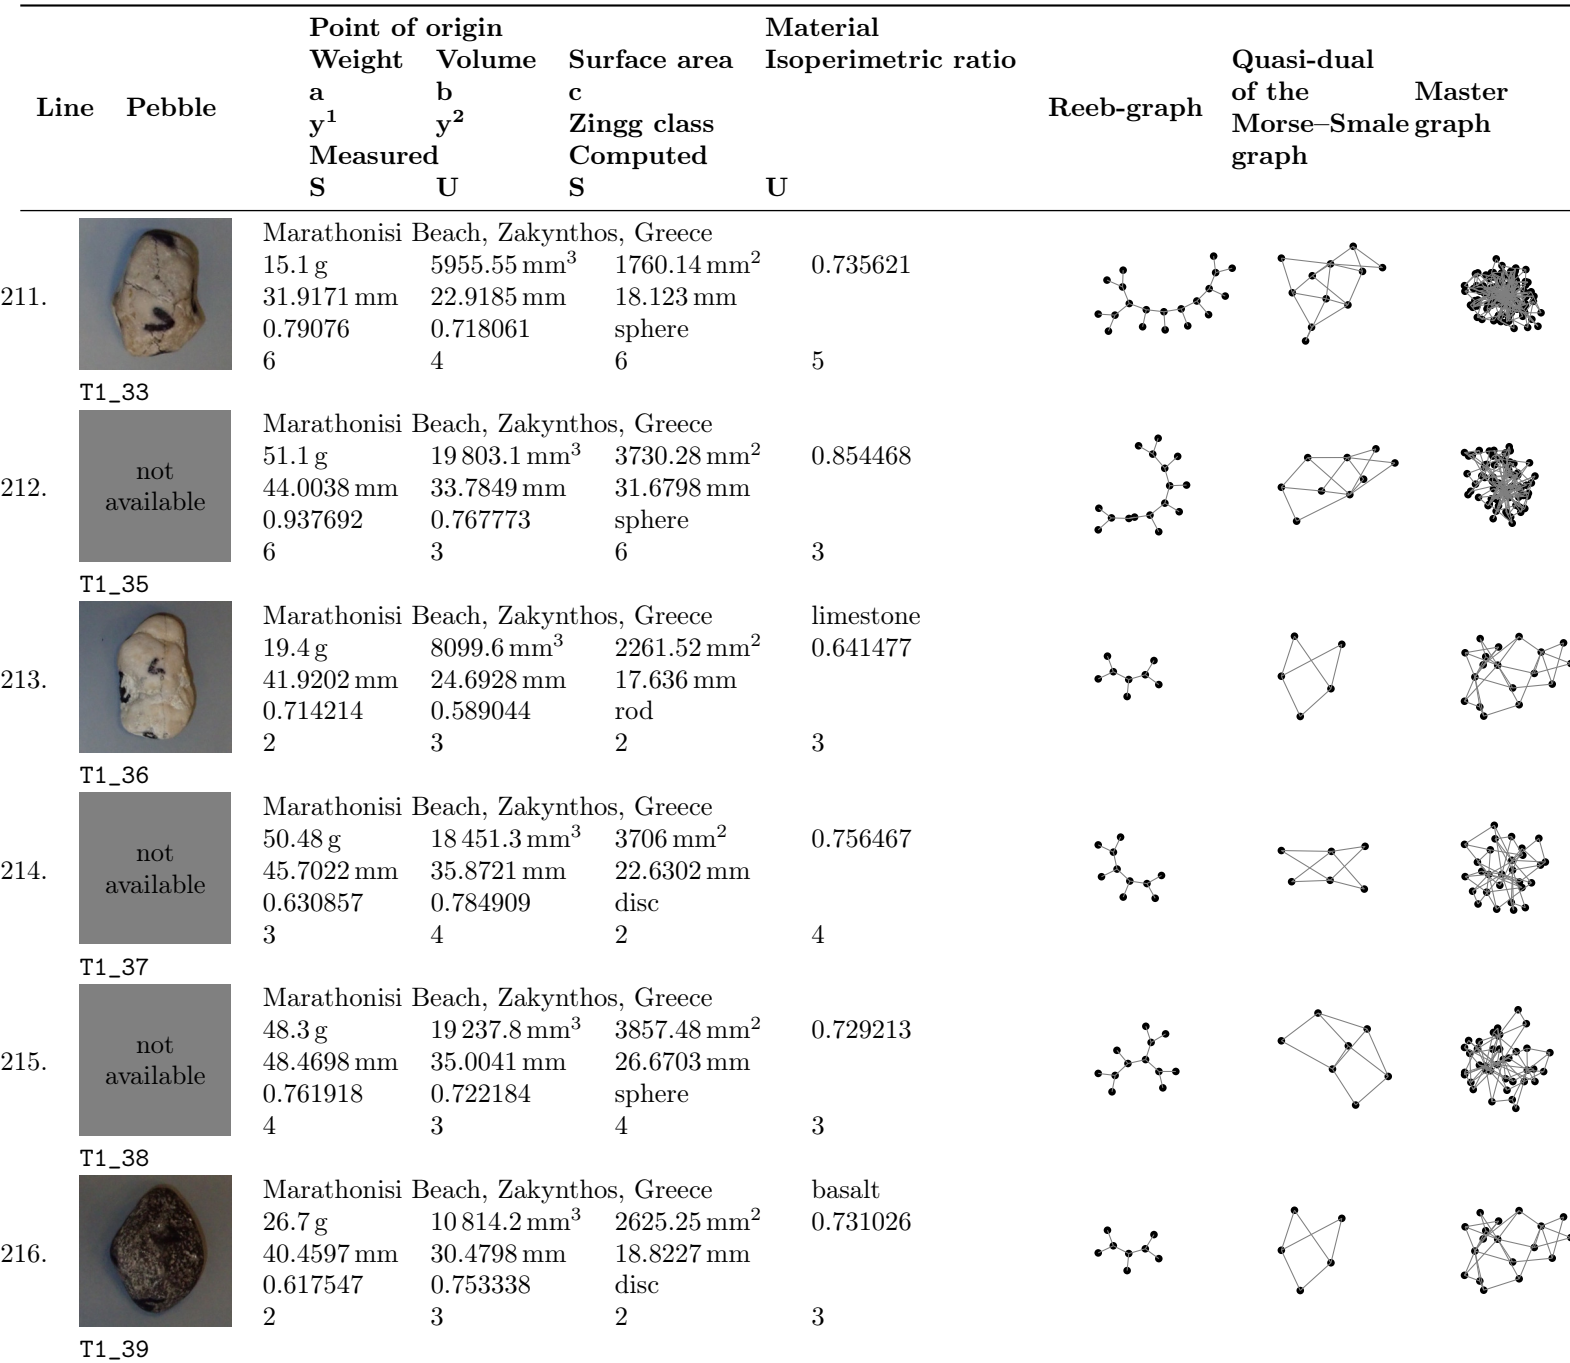   | 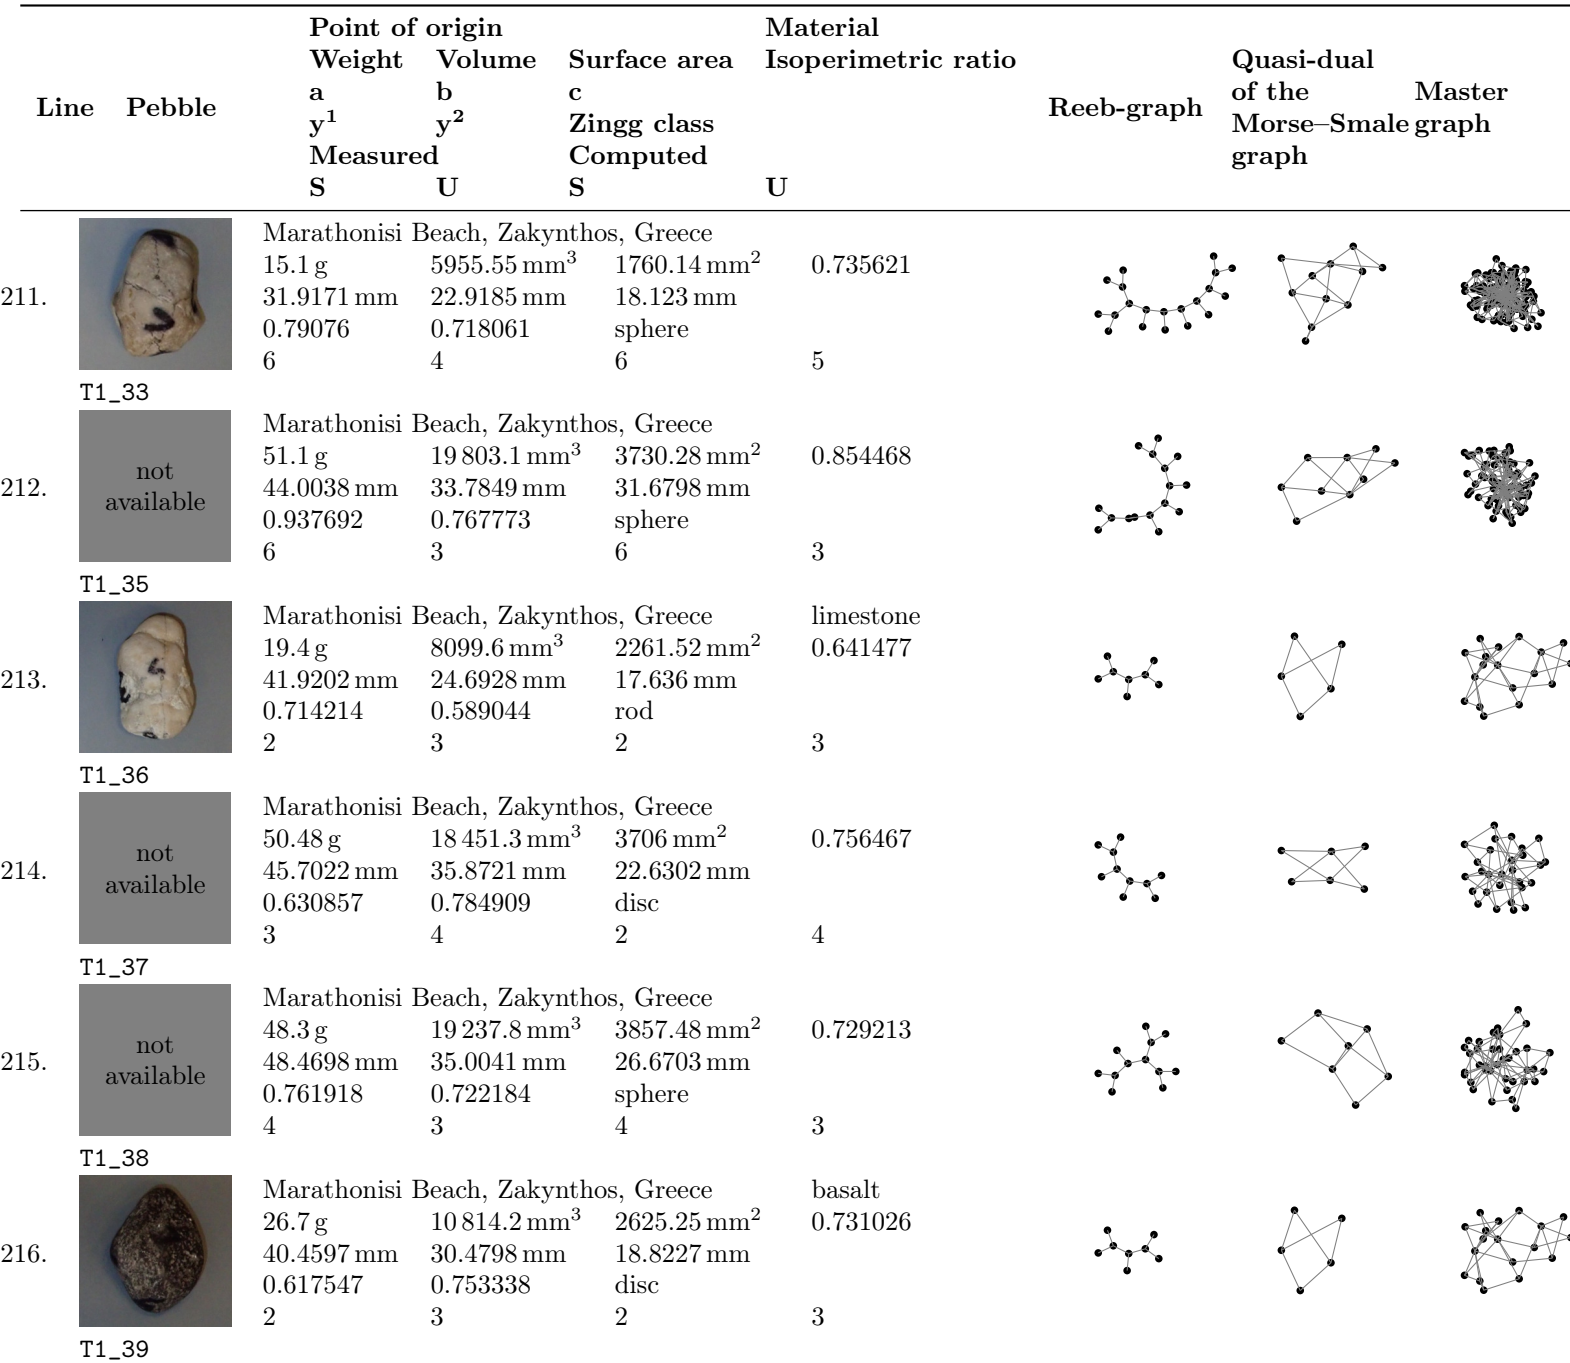   | 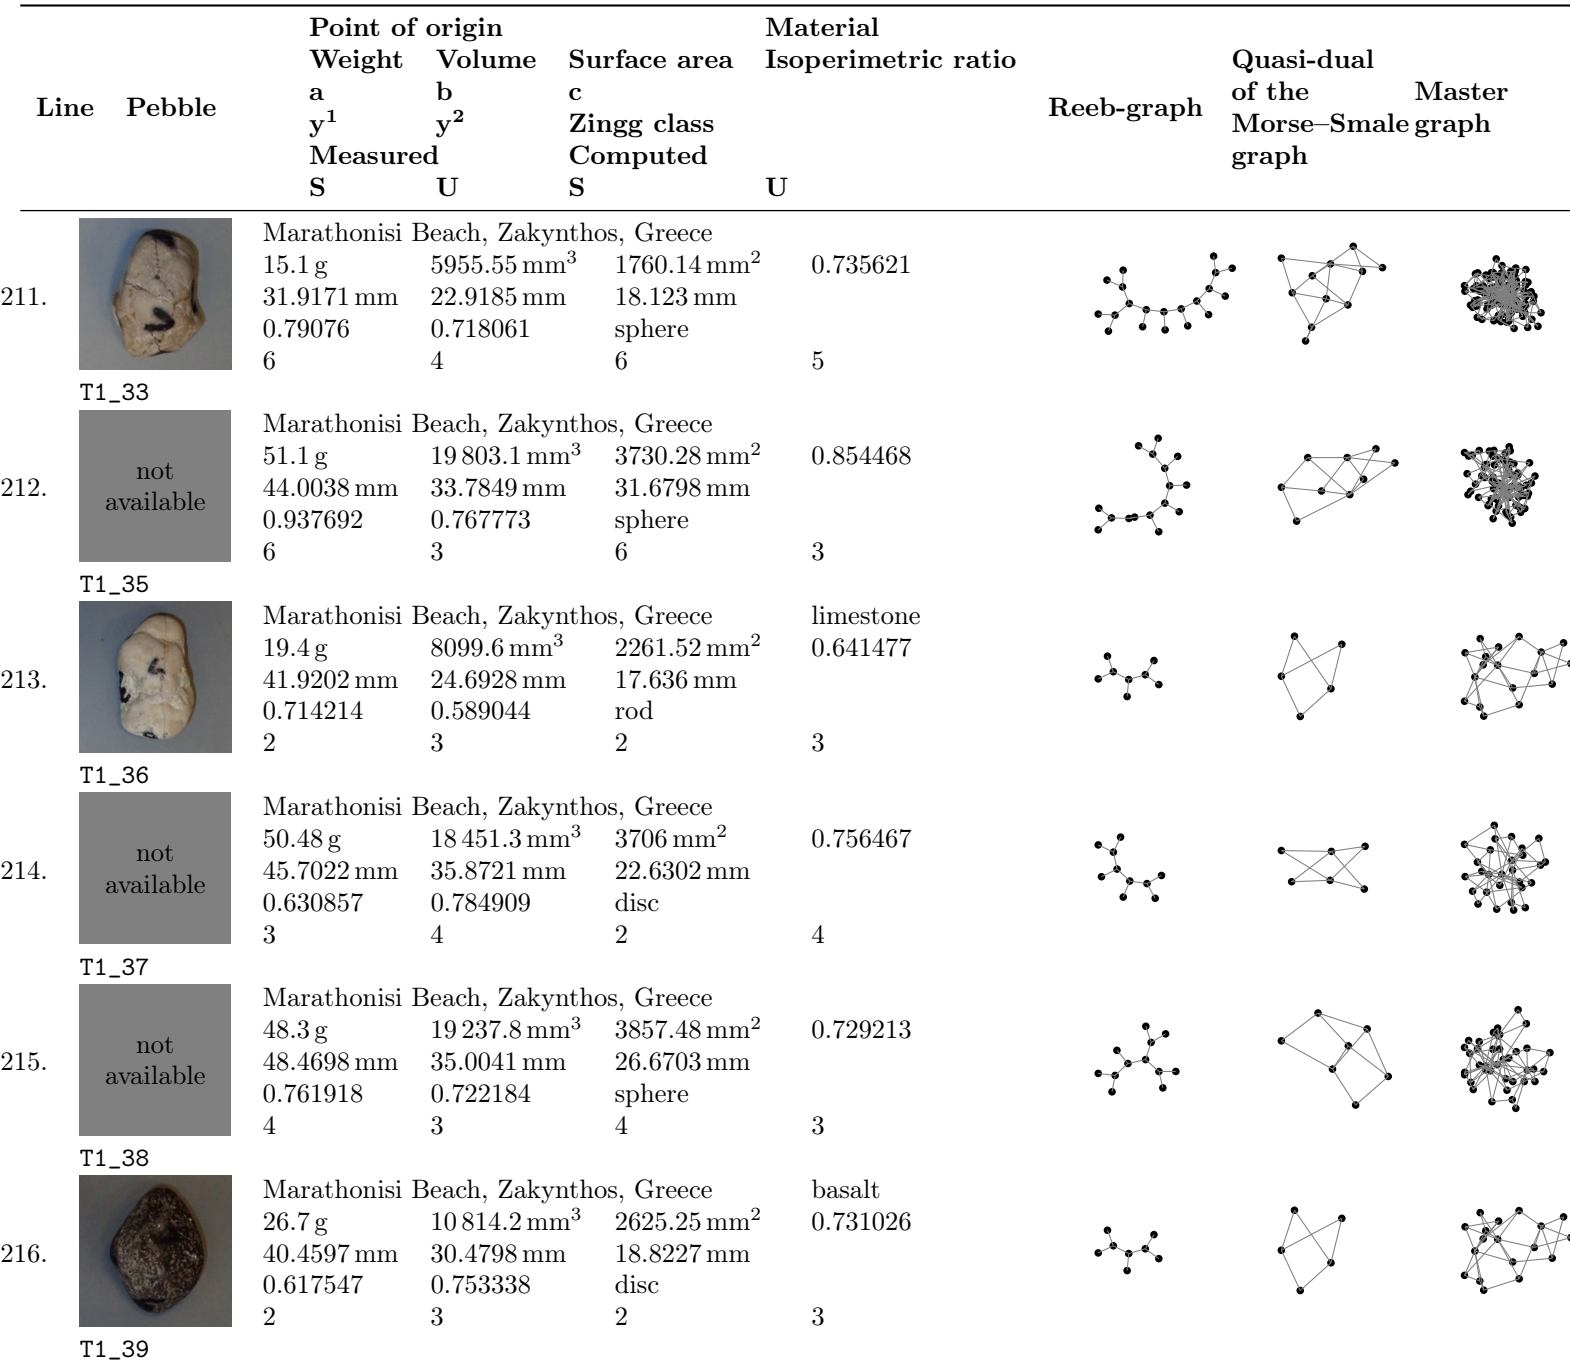   |
|      | T1_33                                                                               |                                      |                          |                         |                     |                                                                                       |                                                                                       |                                                                                       |
| 212. | 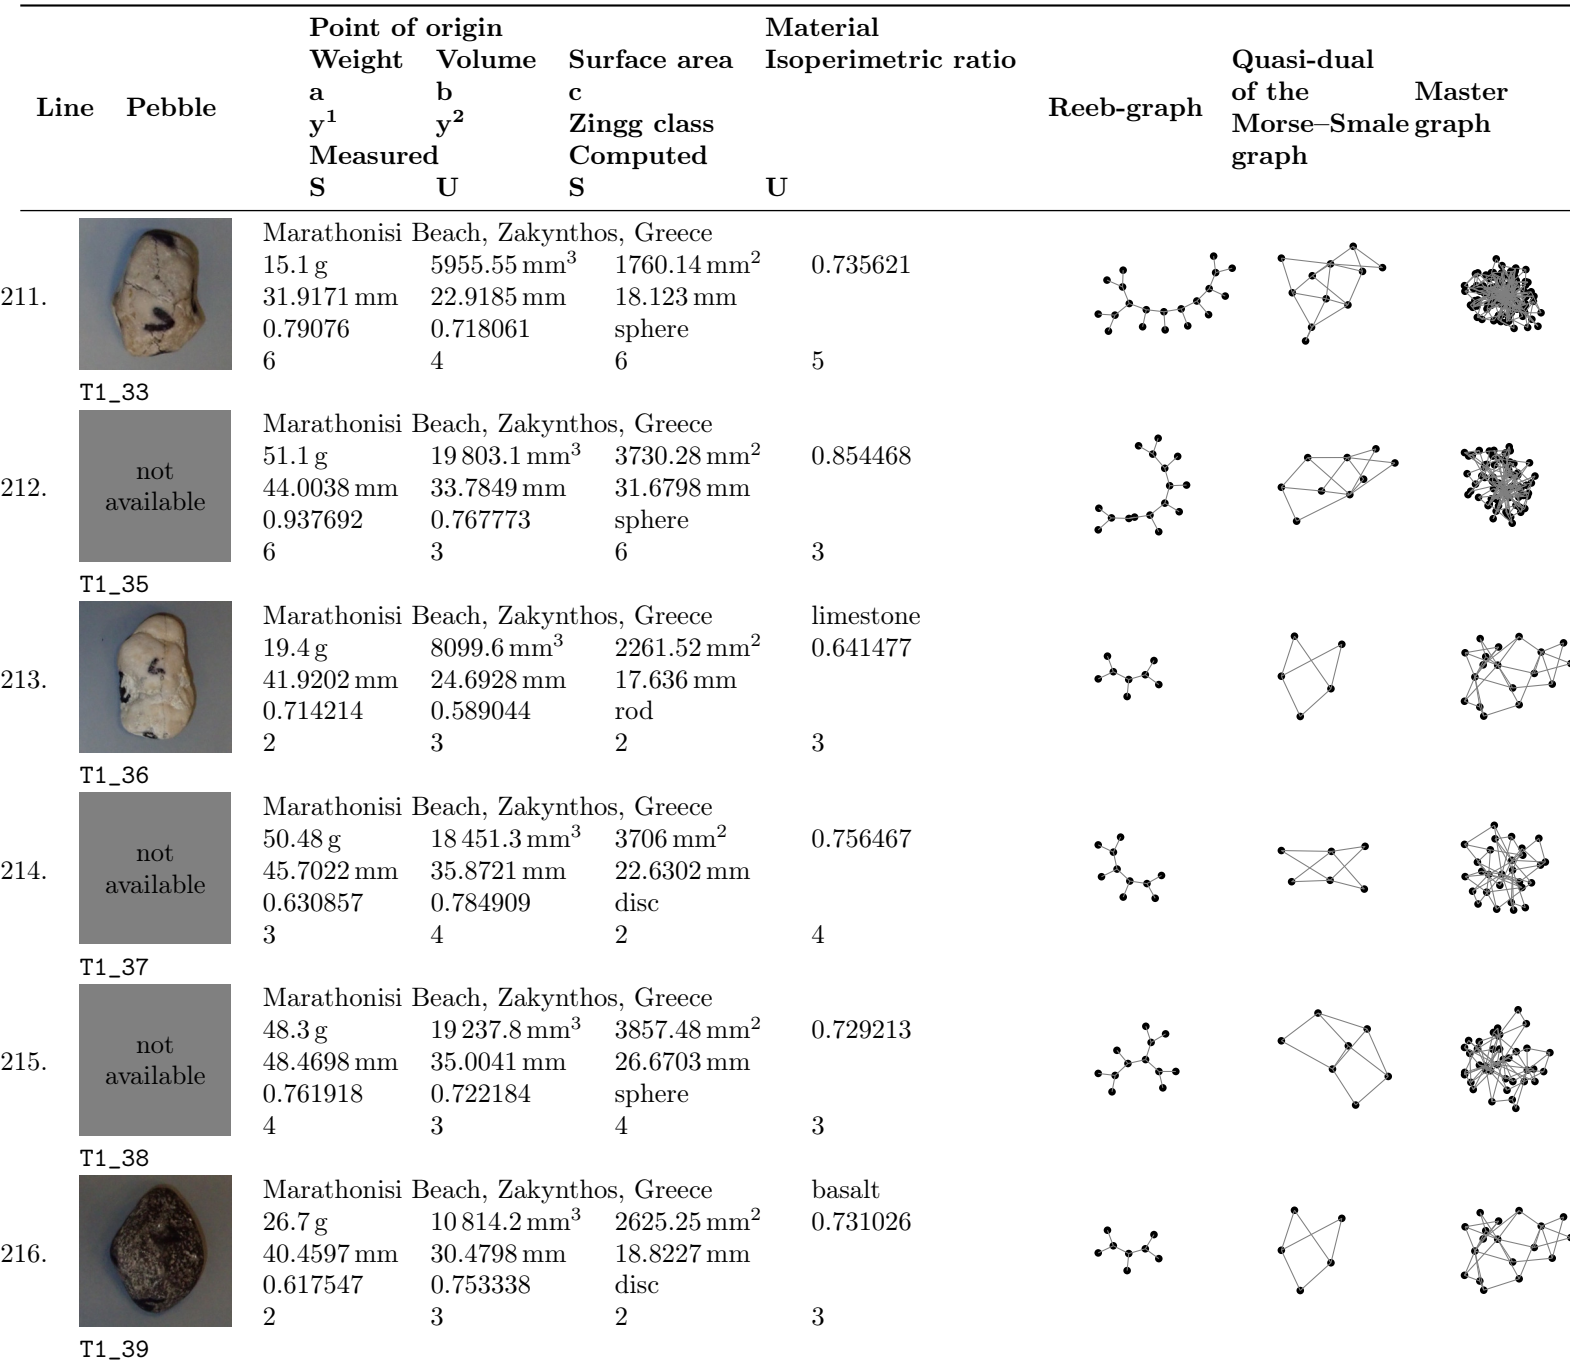   | Marathonisi Beach, Zakynthos, Greece |                          |                         |                     |                                                                                       |                                                                                       |                                                                                       |
|      |                                                                                     | 51.1 g                               | 19 803.1 mm <sup>3</sup> | 3730.28 mm <sup>2</sup> | 0.854468            |                                                                                       |                                                                                       |                                                                                       |
|      |                                                                                     | 44.0038 mm                           | 33.7849 mm               | 31.6798 mm              |                     |                                                                                       |                                                                                       |                                                                                       |
|      |                                                                                     | 0.937692                             | 0.767773                 | sphere                  |                     |                                                                                       |                                                                                       |                                                                                       |
|      |                                                                                     | 6                                    | 3                        | 6                       | 3                   | 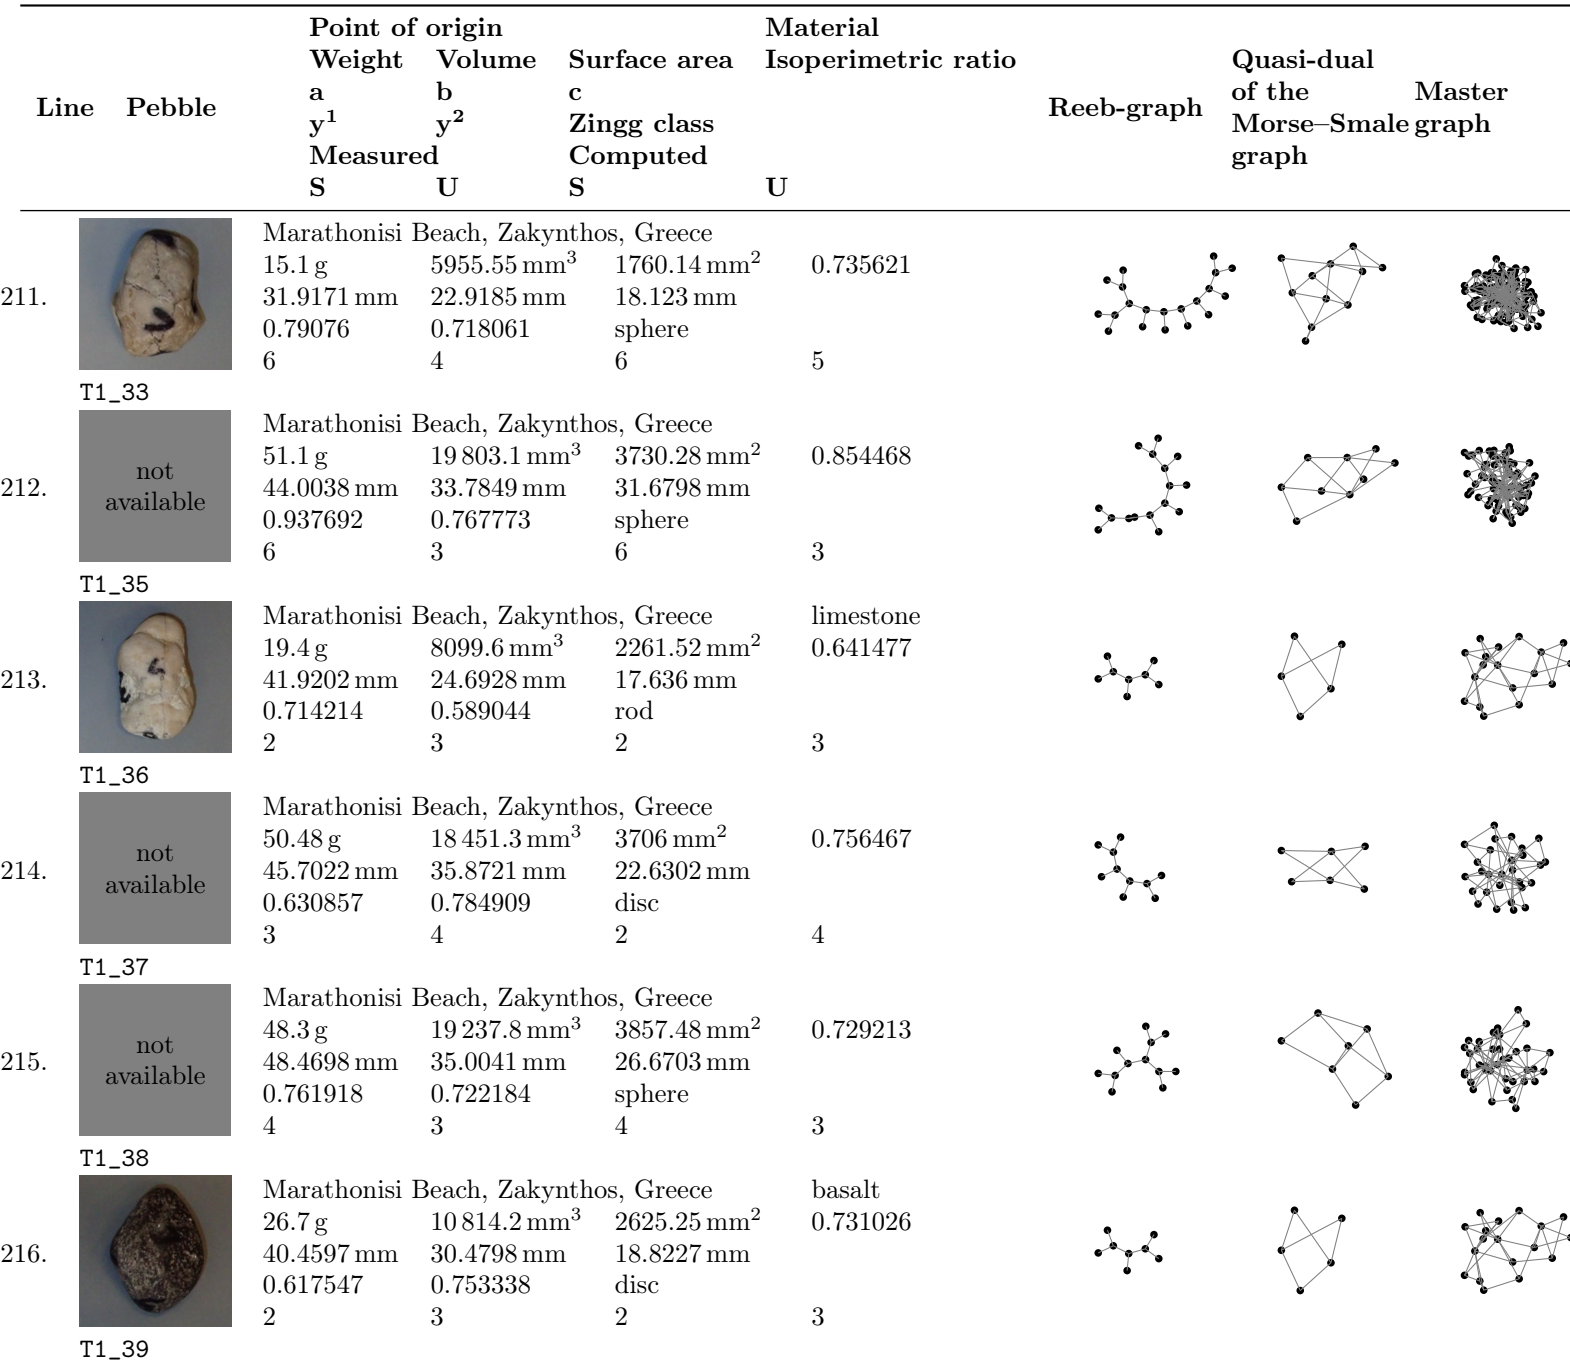   | 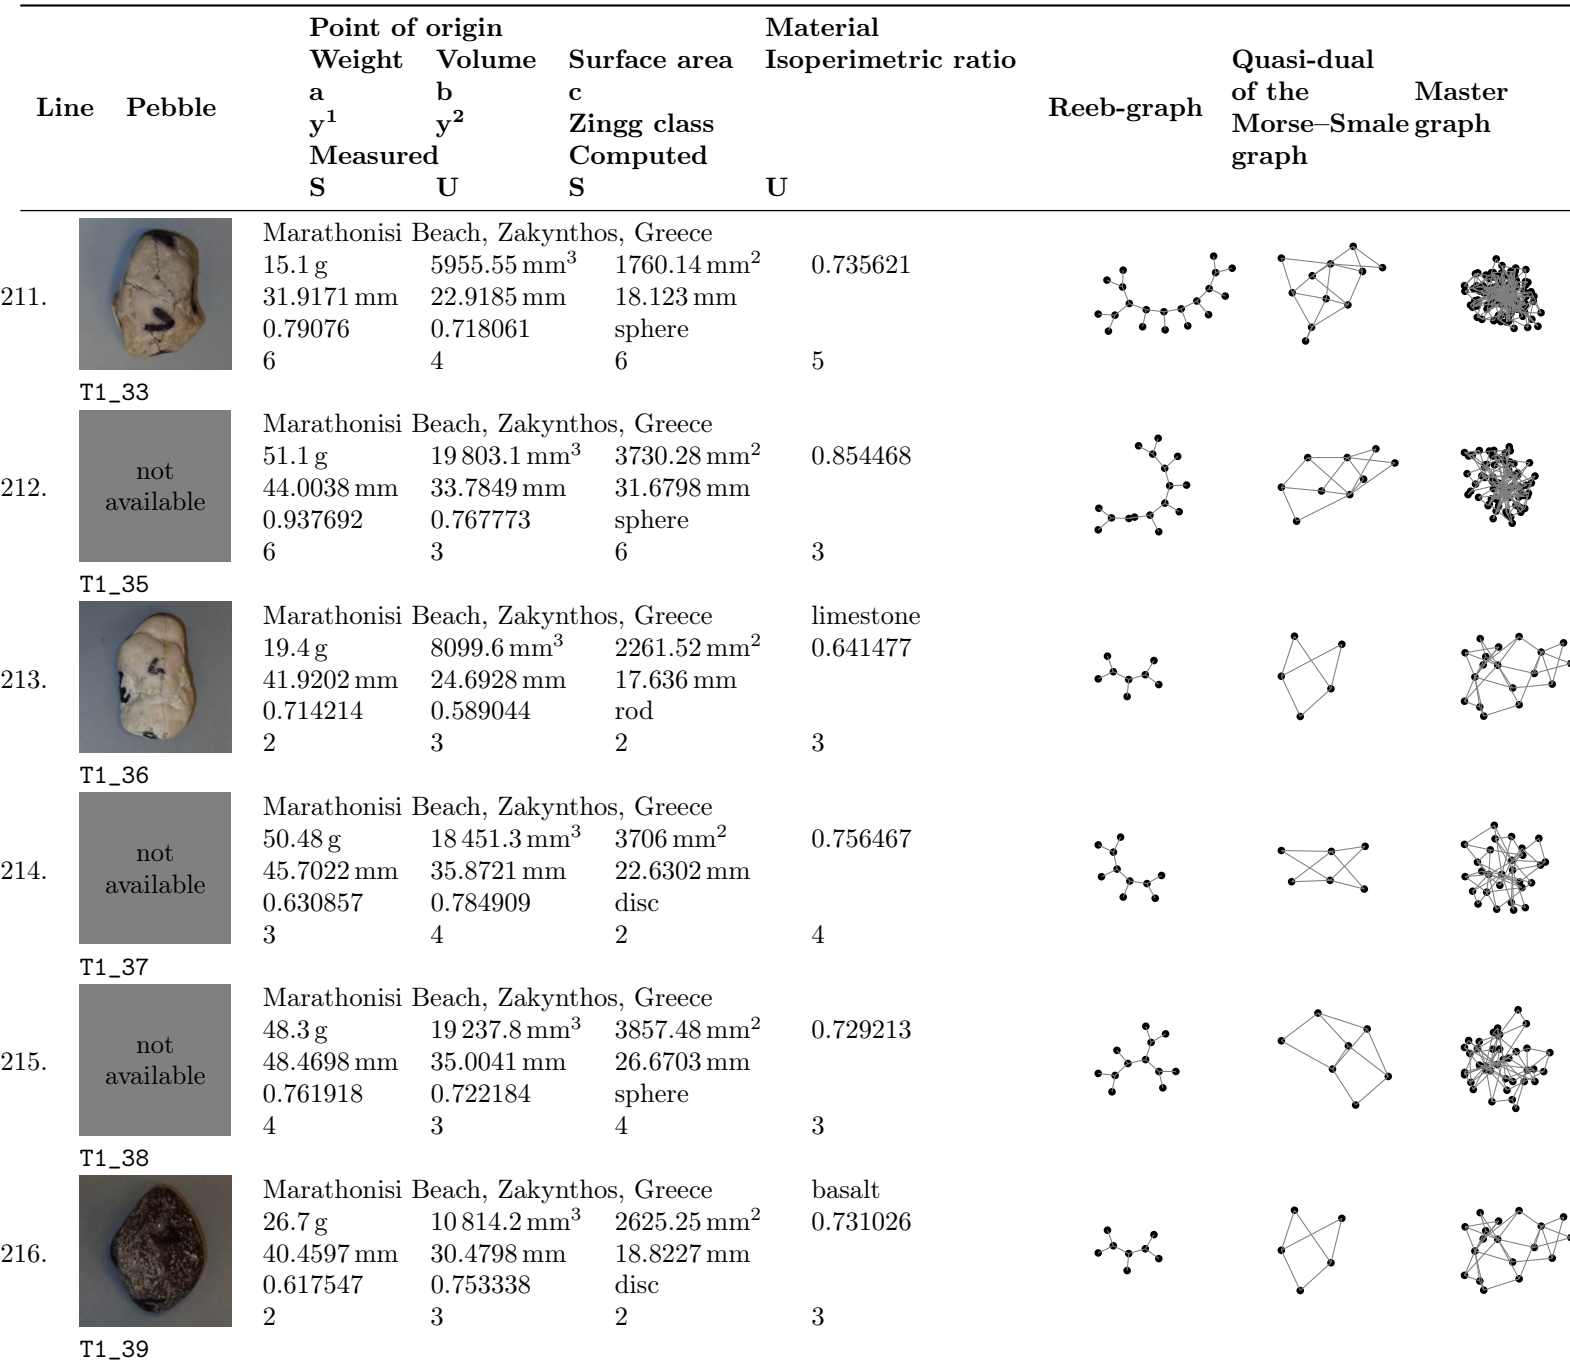   | 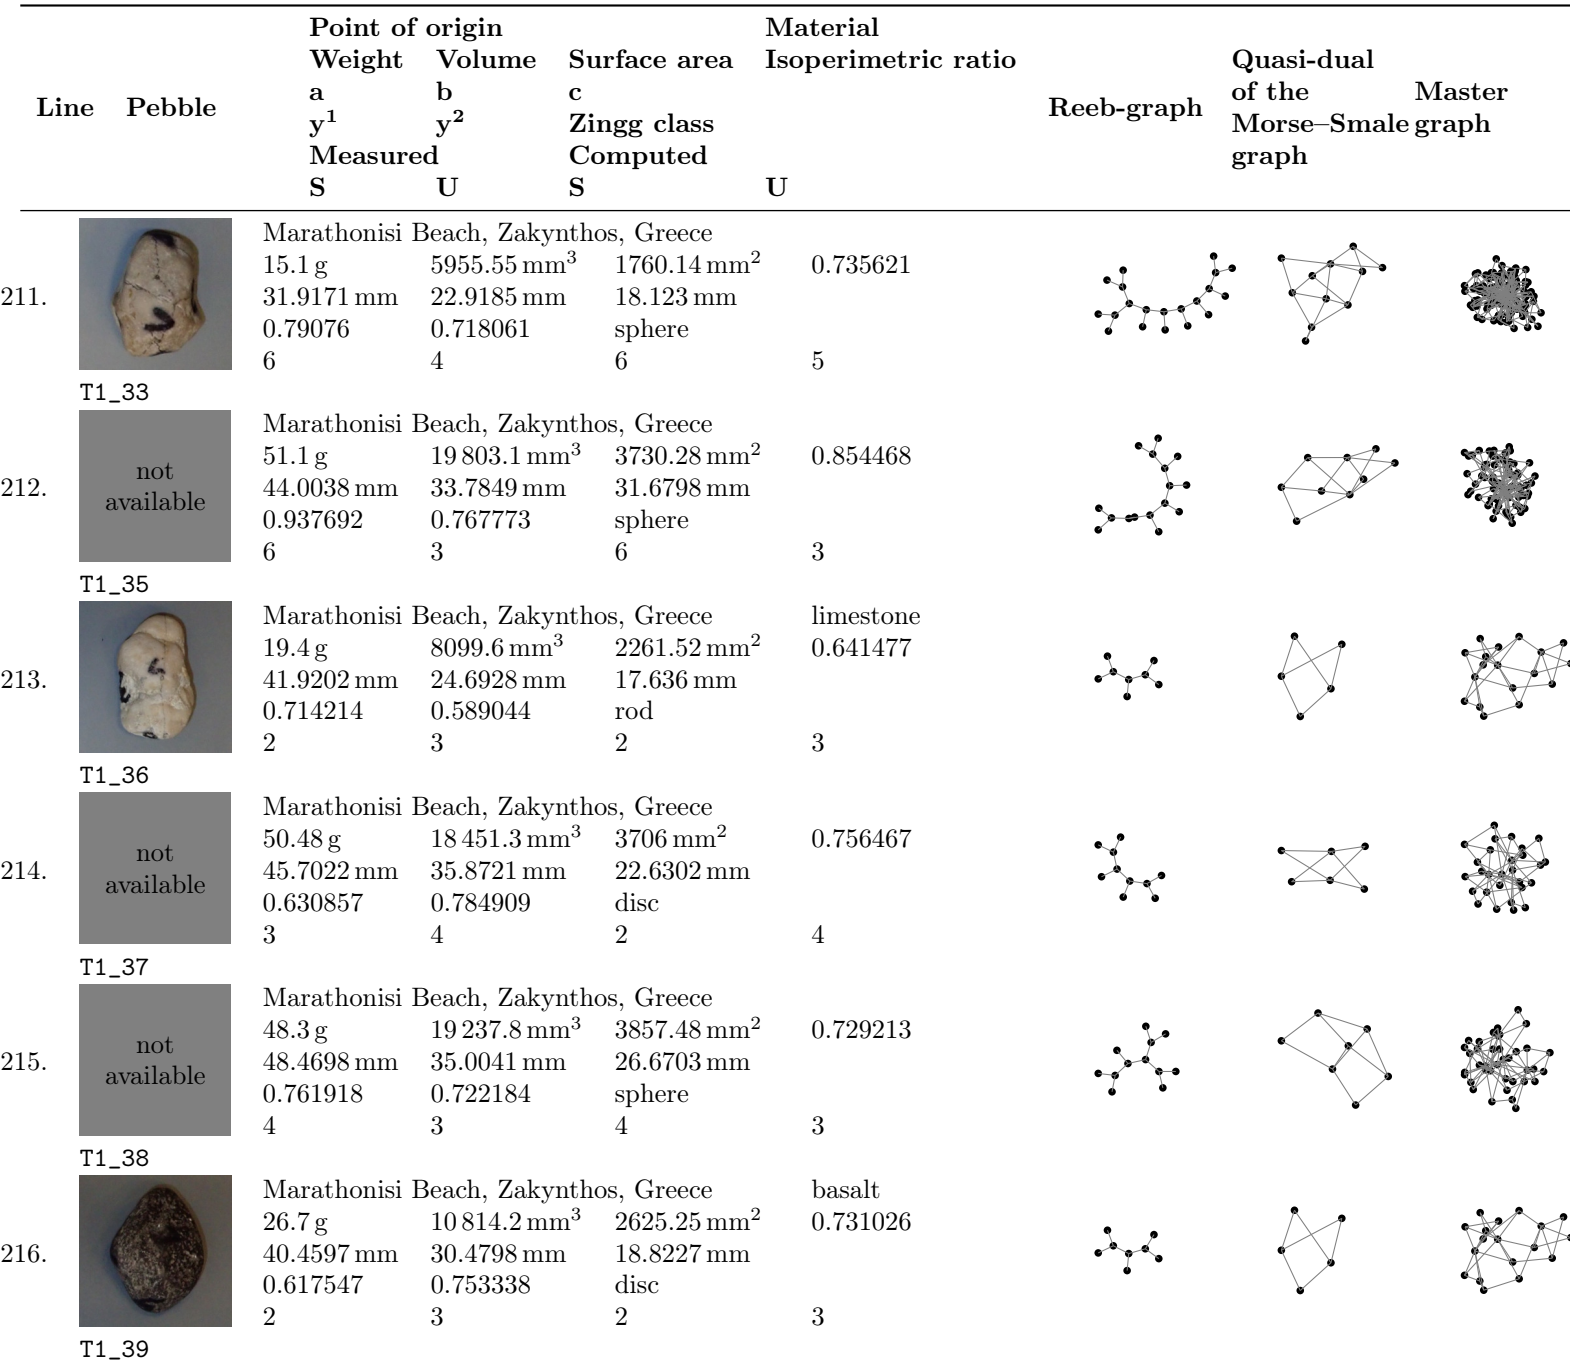   |
|      | T1_35                                                                               |                                      |                          |                         |                     |                                                                                       |                                                                                       |                                                                                       |
| 213. | 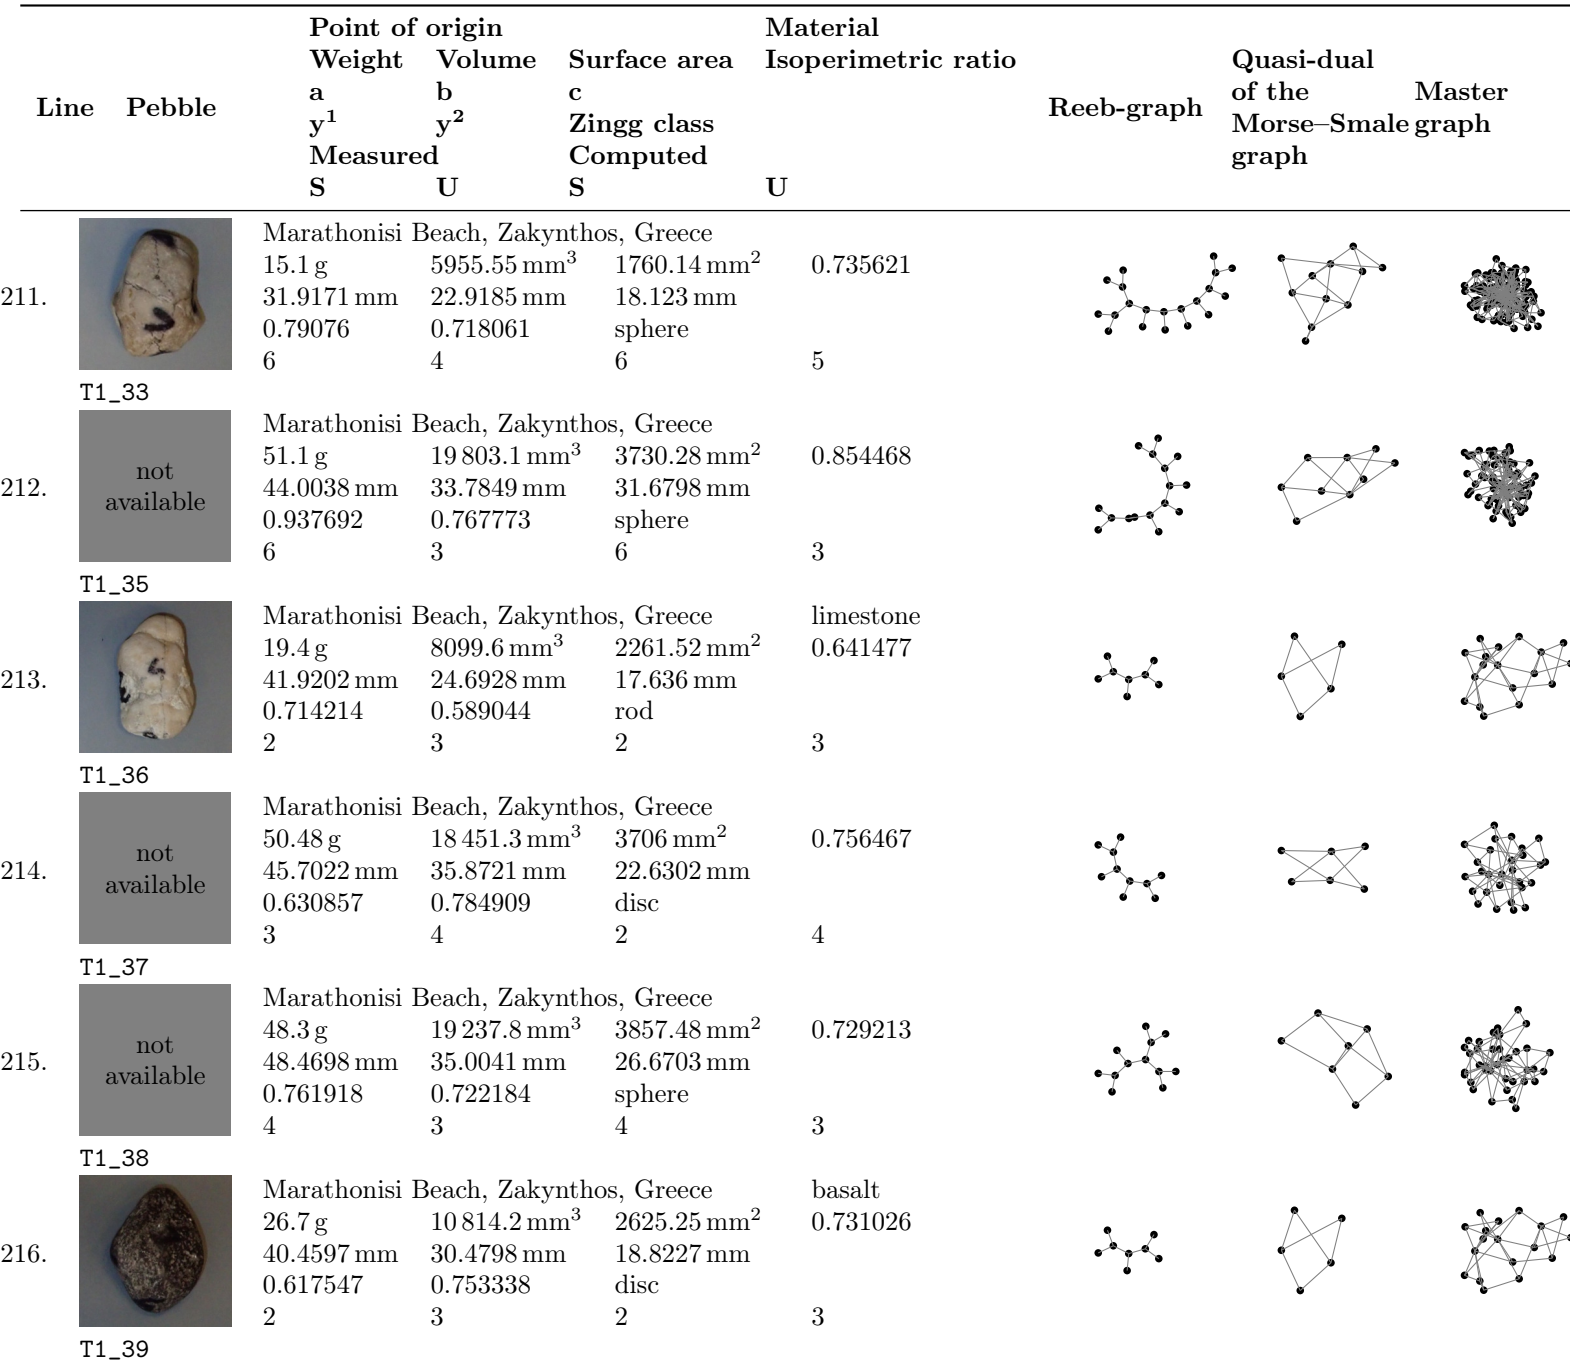   | Marathonisi Beach, Zakynthos, Greece |                          |                         | limestone           |                                                                                       |                                                                                       |                                                                                       |
|      |                                                                                     | 19.4 g                               | 8099.6 mm <sup>3</sup>   | 2261.52 mm <sup>2</sup> | 0.641477            |                                                                                       |                                                                                       |                                                                                       |
|      |                                                                                     | 41.9202 mm                           | 24.6928 mm               | 17.636 mm               |                     |                                                                                       |                                                                                       |                                                                                       |
|      |                                                                                     | 0.714214                             | 0.589044                 | rod                     |                     |                                                                                       |                                                                                       |                                                                                       |
|      |                                                                                     | 2                                    | 3                        | 2                       | 3                   | 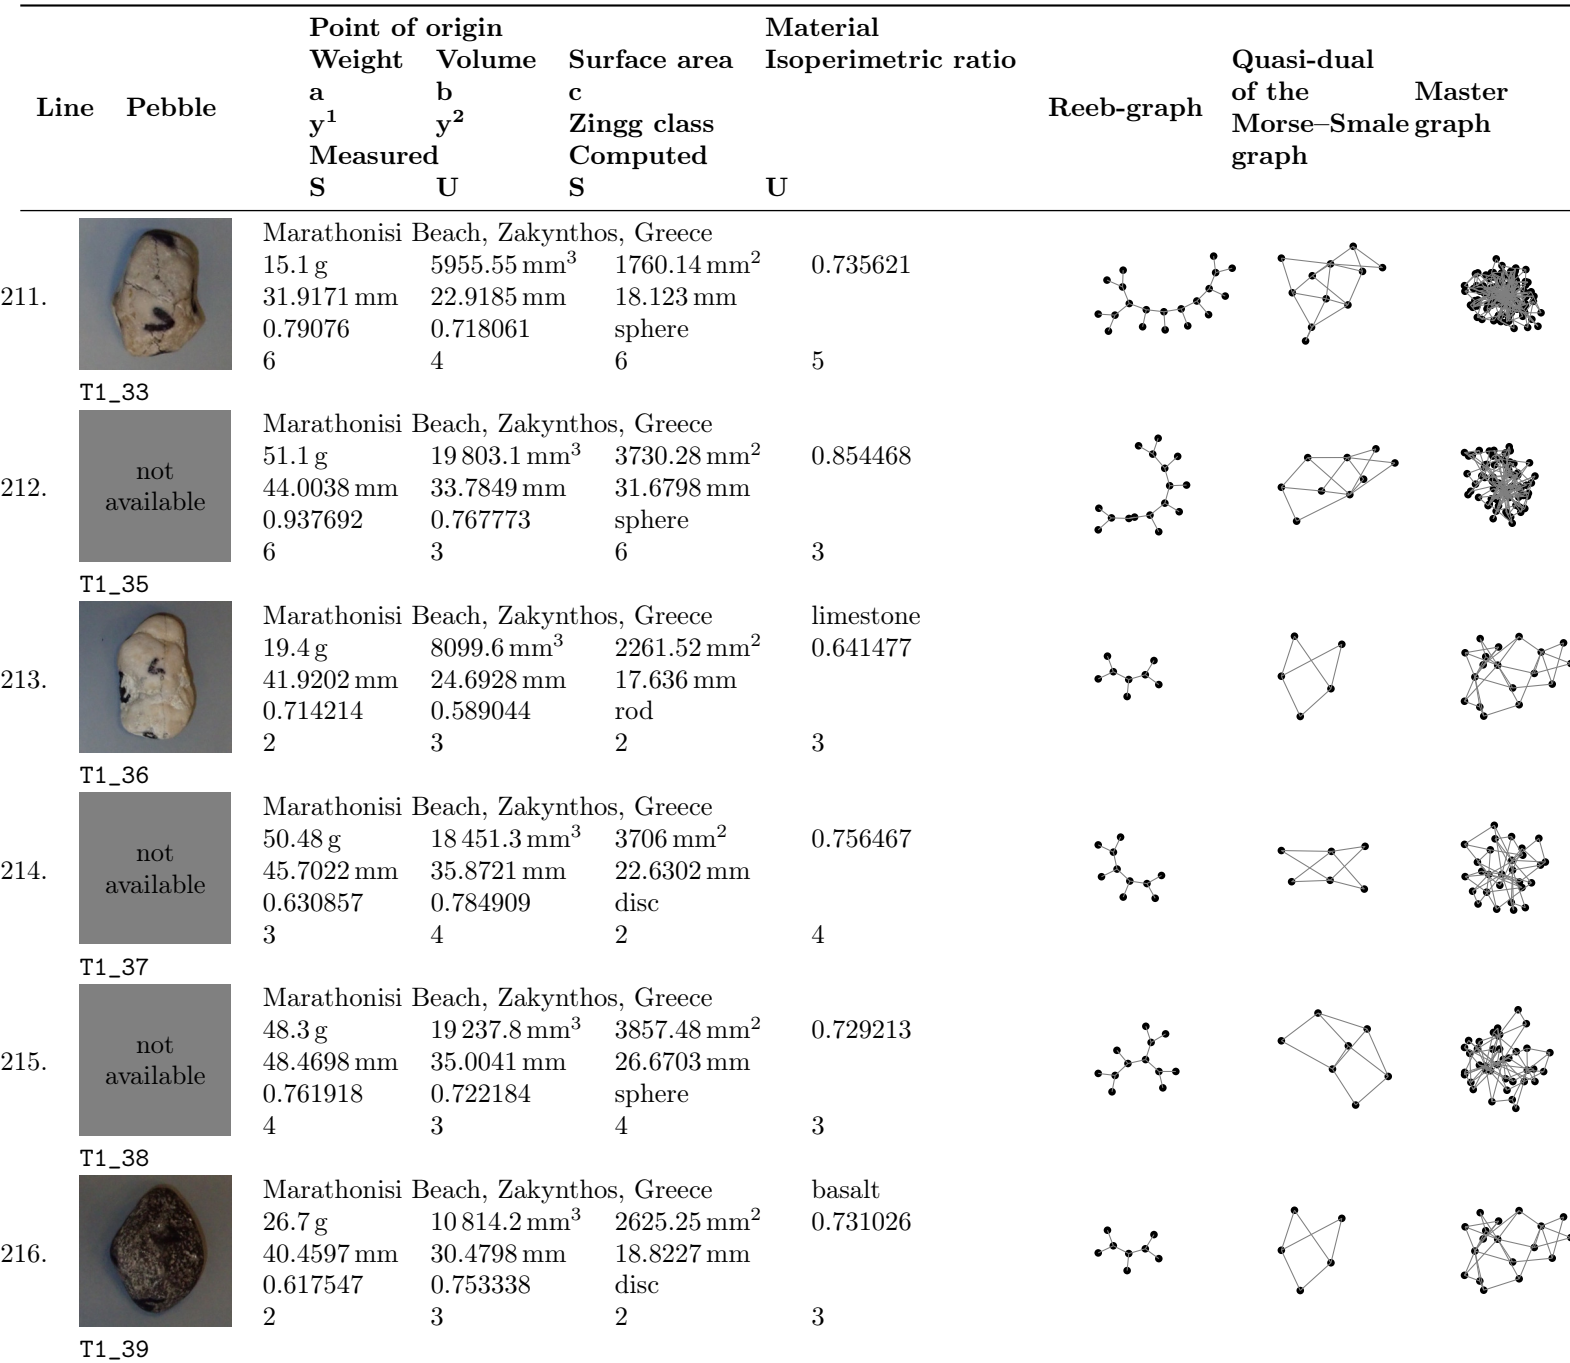   | 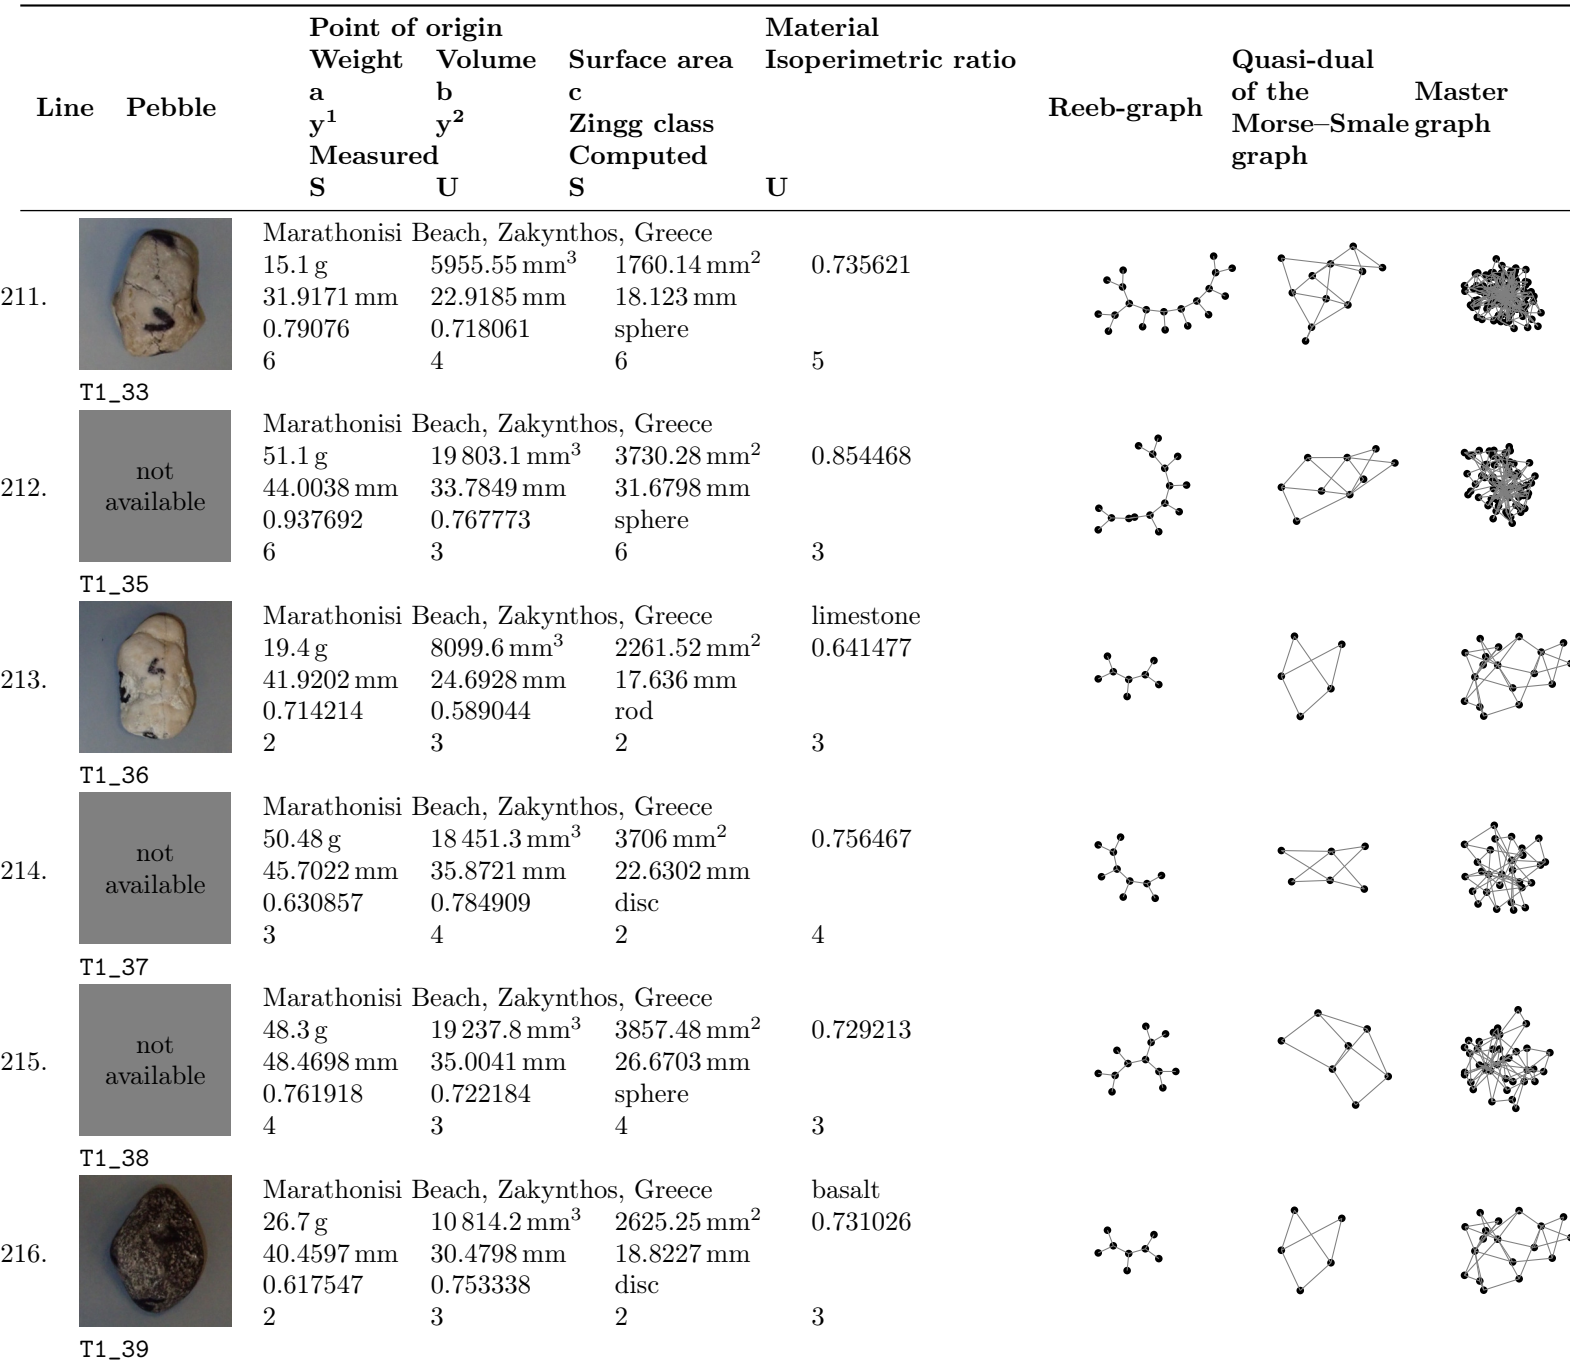   | 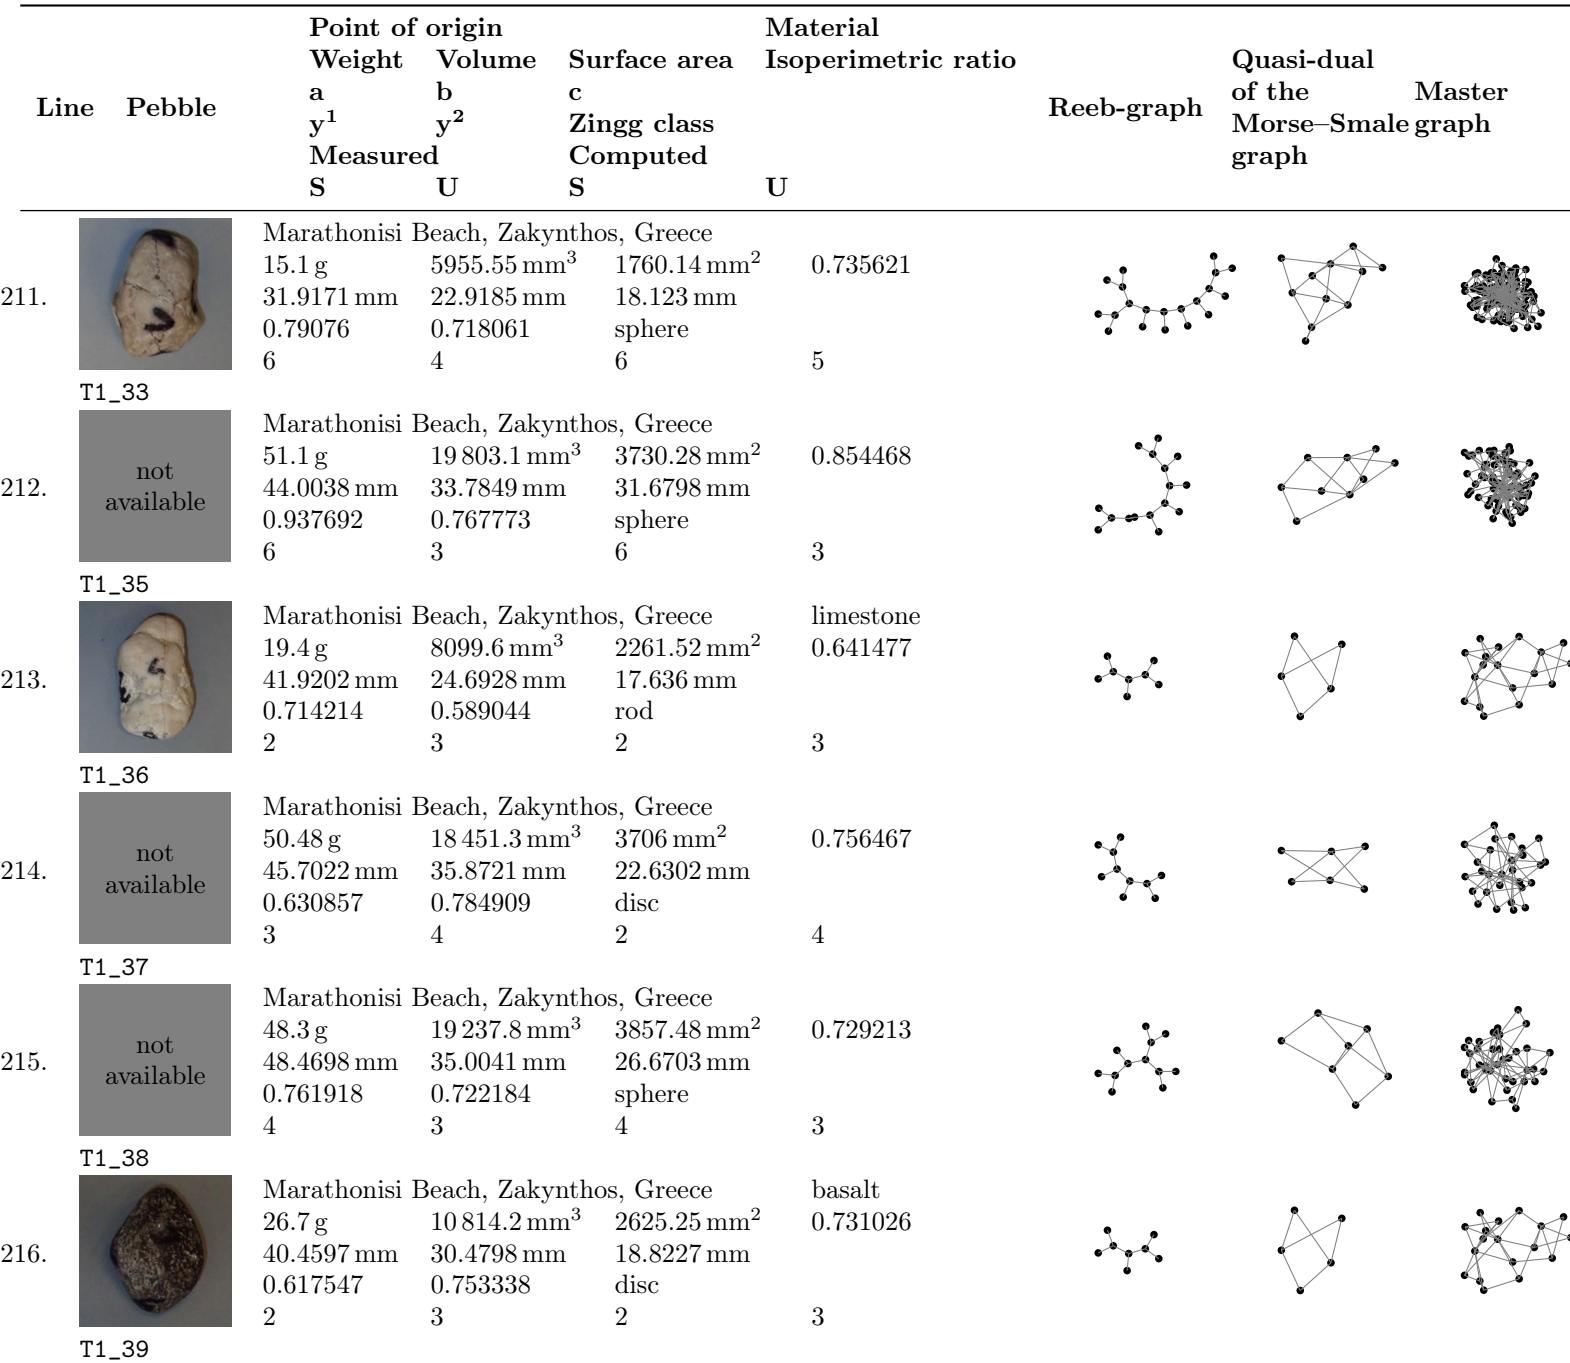   |
|      | T1_36                                                                               |                                      |                          |                         |                     |                                                                                       |                                                                                       |                                                                                       |
| 214. | 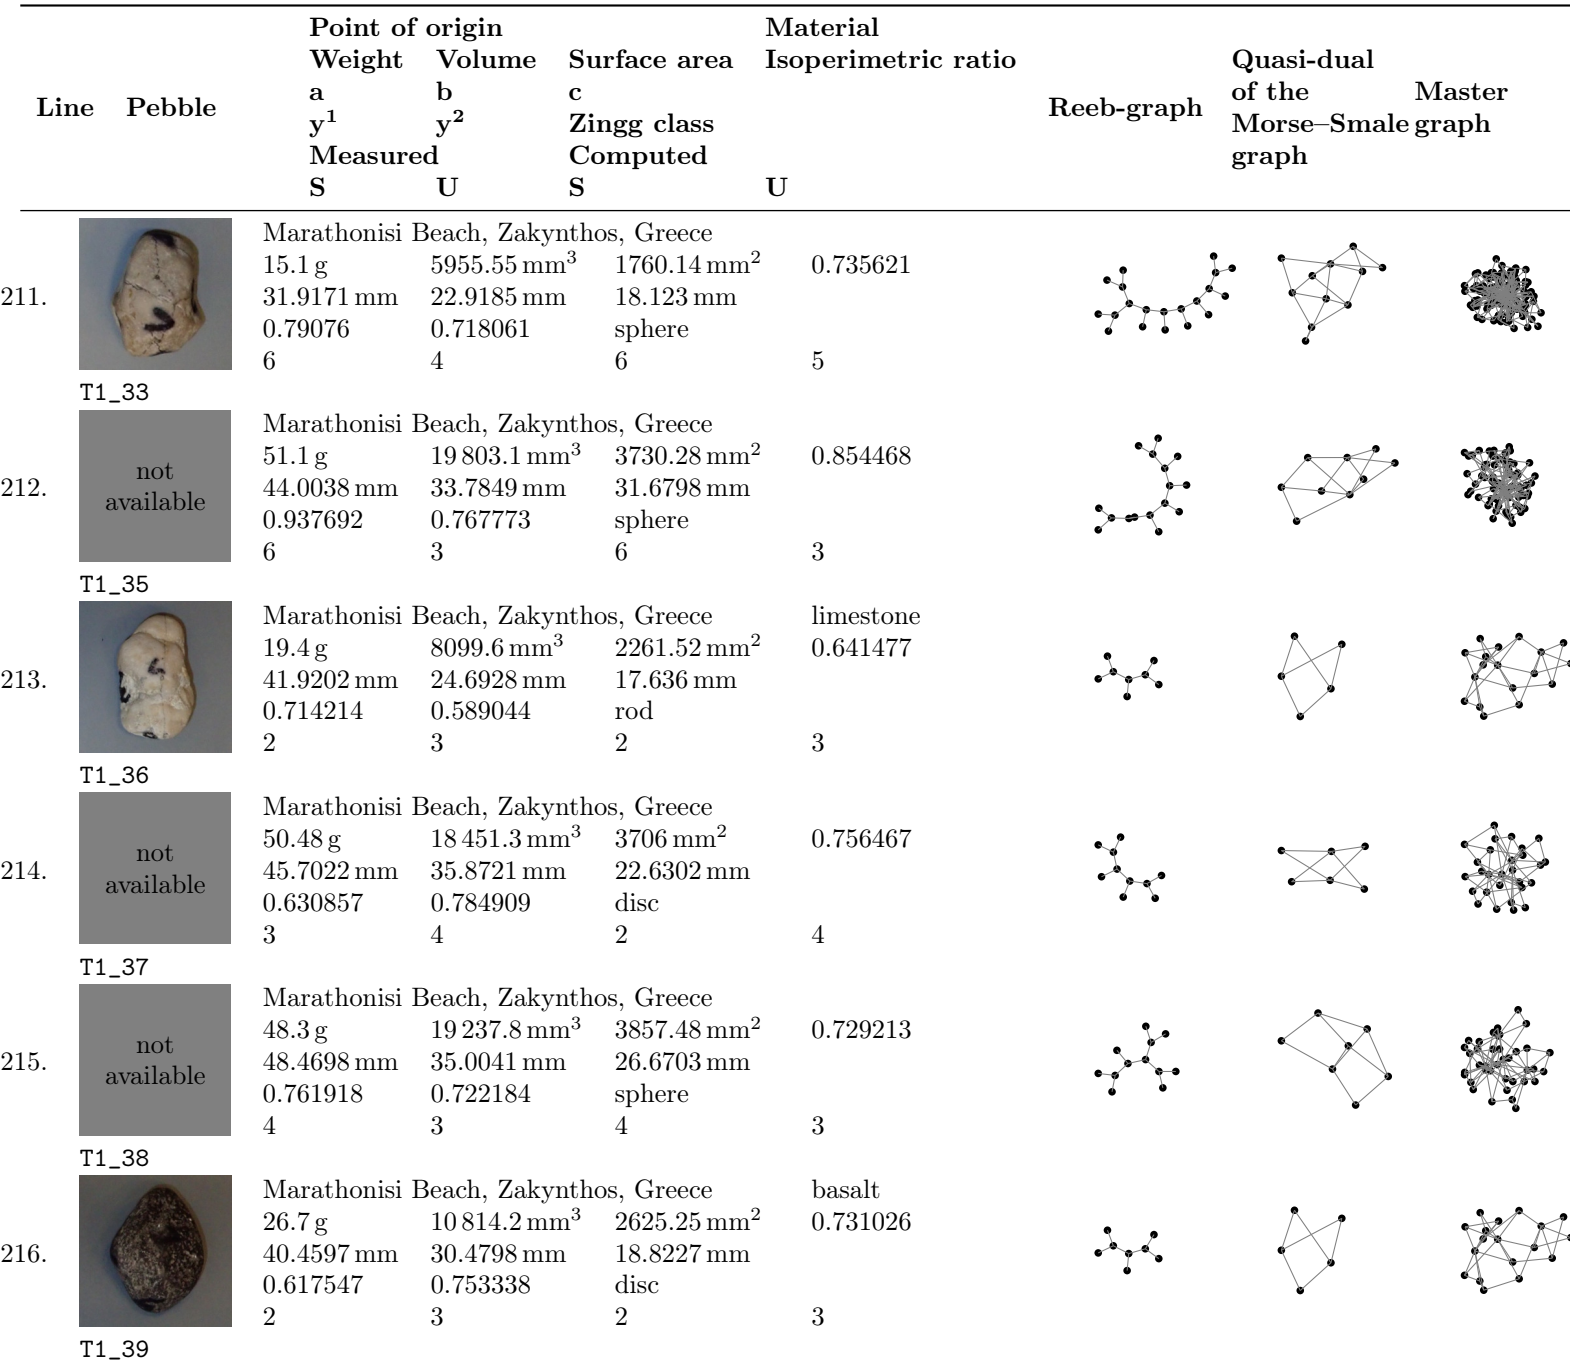  | Marathonisi Beach, Zakynthos, Greece |                          |                         |                     |                                                                                       |                                                                                       |                                                                                       |
|      |                                                                                     | 50.48 g                              | 18 451.3 mm <sup>3</sup> | 3706 mm <sup>2</sup>    | 0.756467            |                                                                                       |                                                                                       |                                                                                       |
|      |                                                                                     | 45.7022 mm                           | 35.8721 mm               | 22.6302 mm              |                     |                                                                                       |                                                                                       |                                                                                       |
|      |                                                                                     | 0.630857                             | 0.784909                 | disc                    |                     |                                                                                       |                                                                                       |                                                                                       |
|      |                                                                                     | 3                                    | 4                        | 2                       | 4                   | 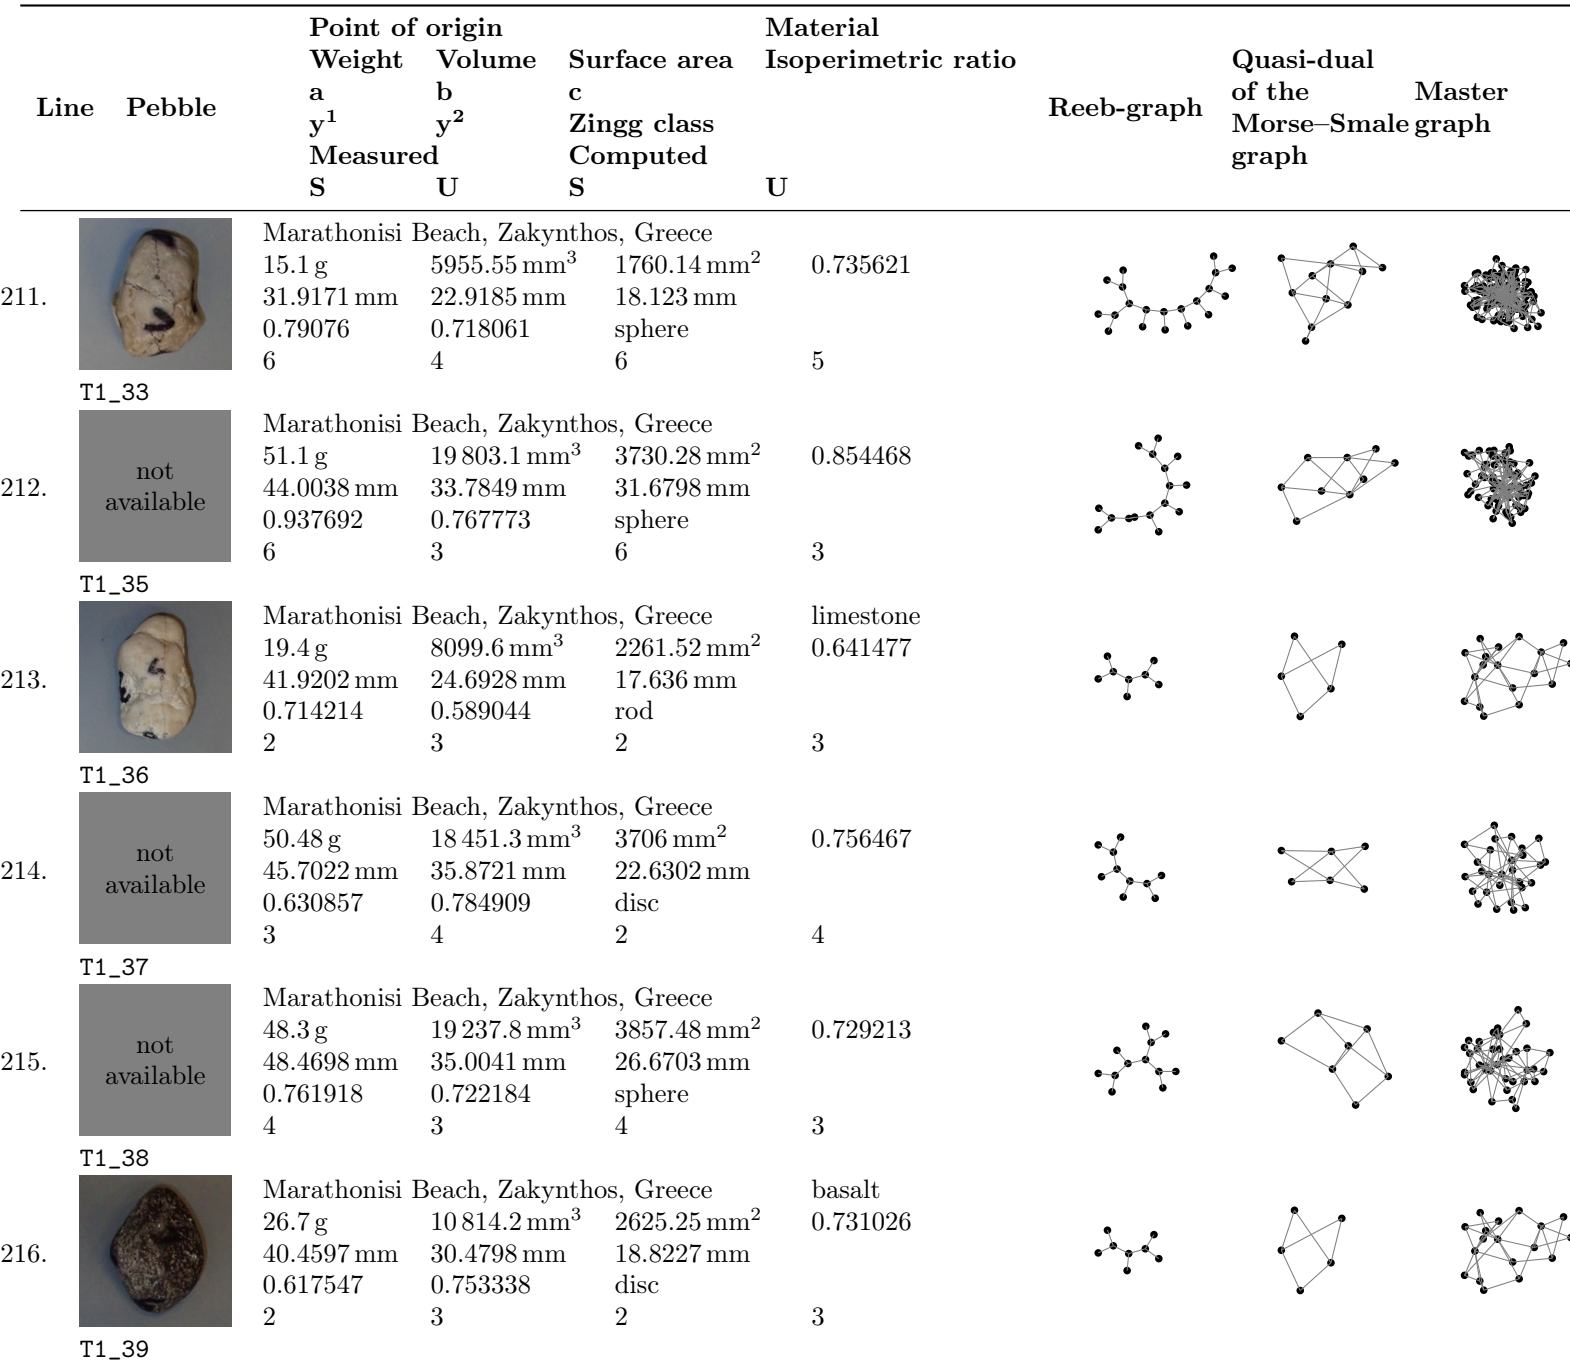  | 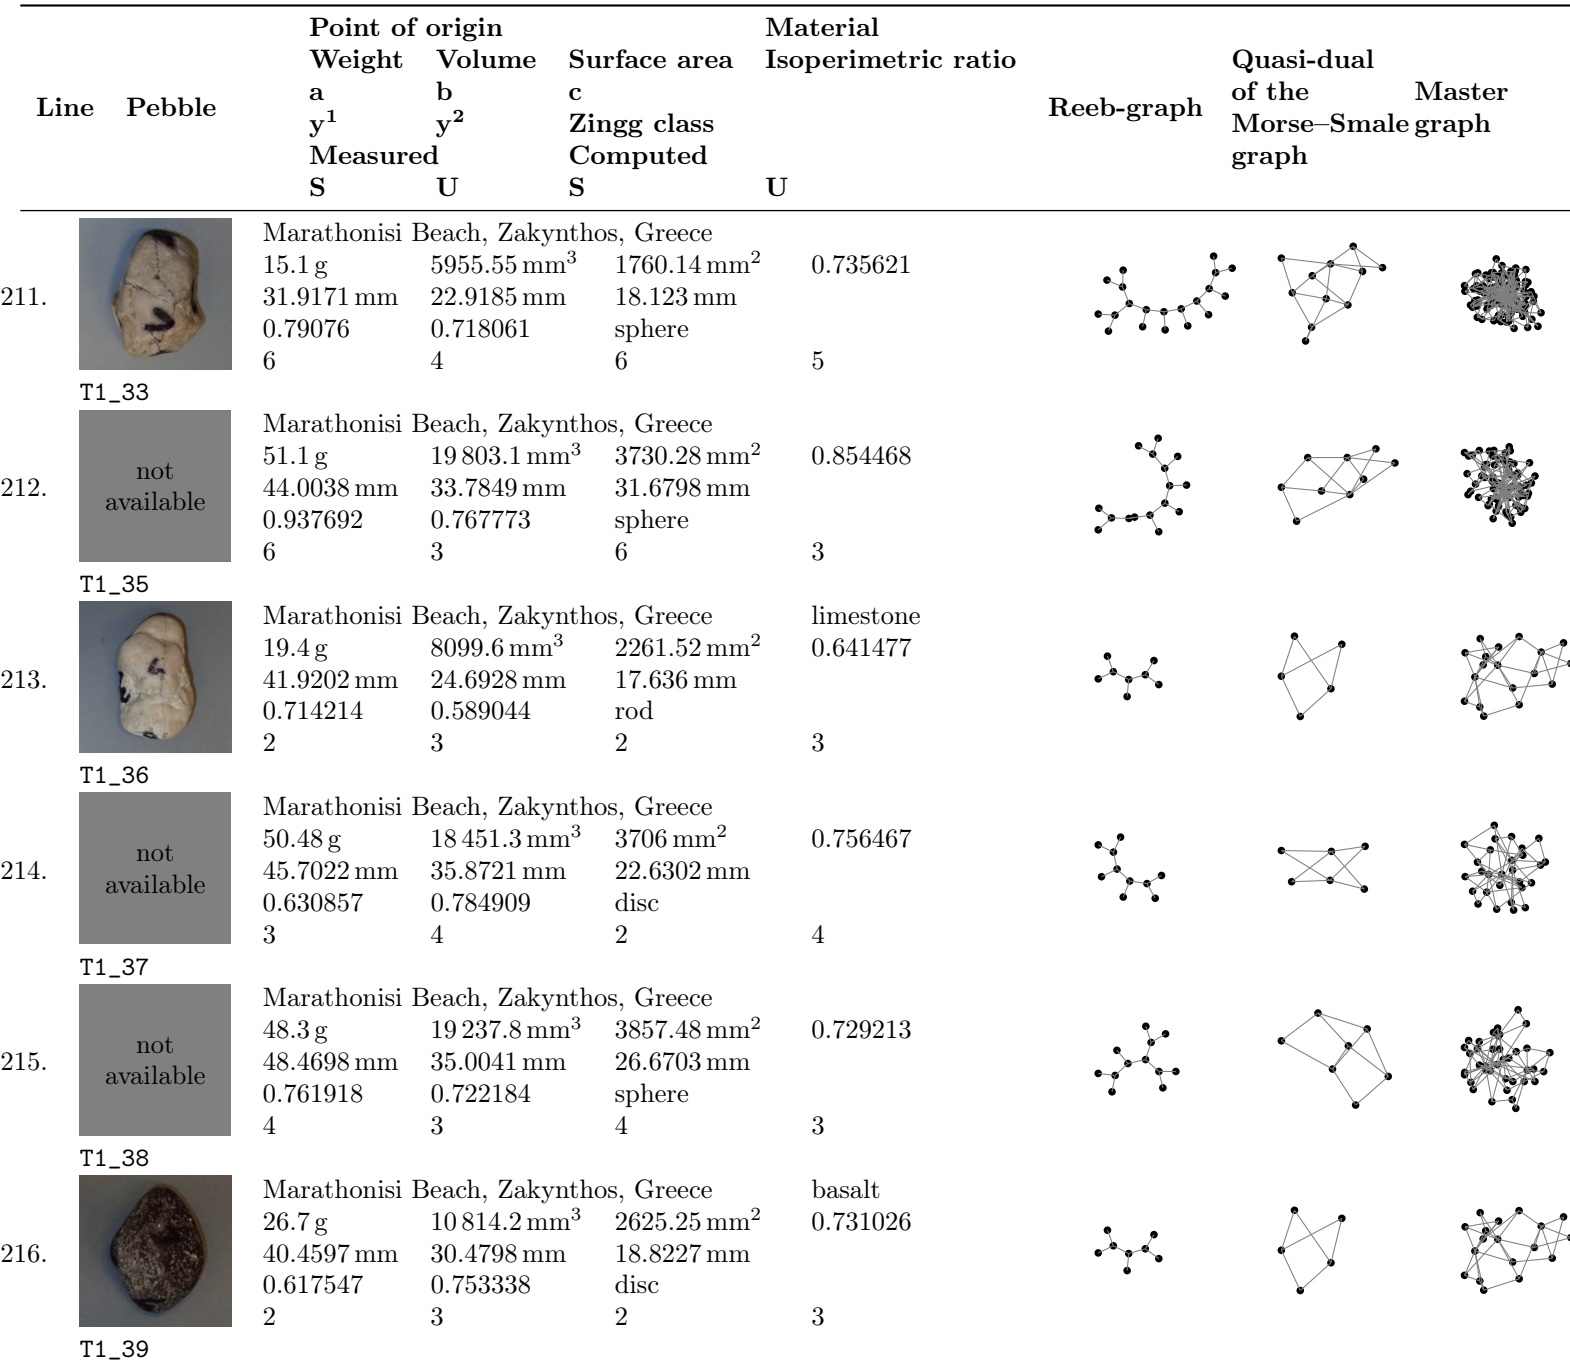  | 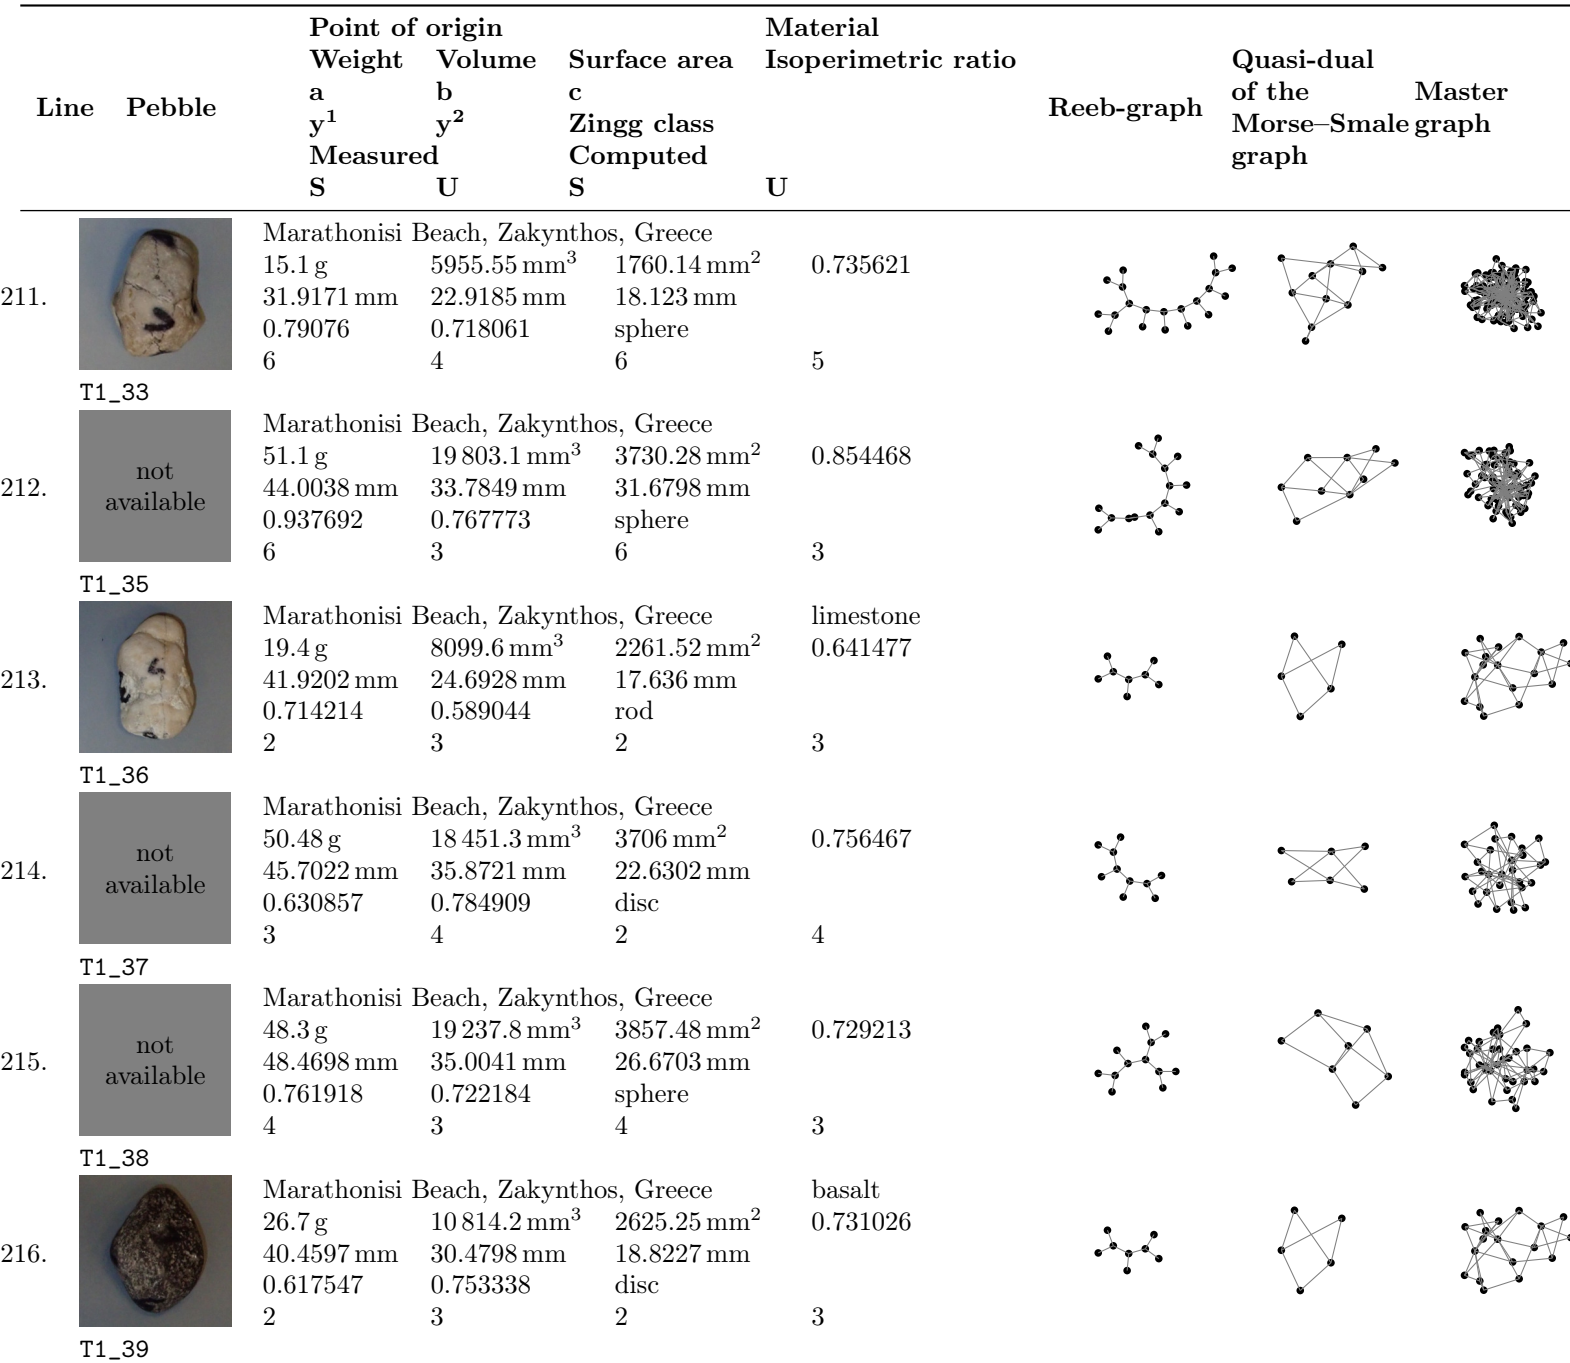  |
|      | T1_37                                                                               |                                      |                          |                         |                     |                                                                                       |                                                                                       |                                                                                       |
| 215. | 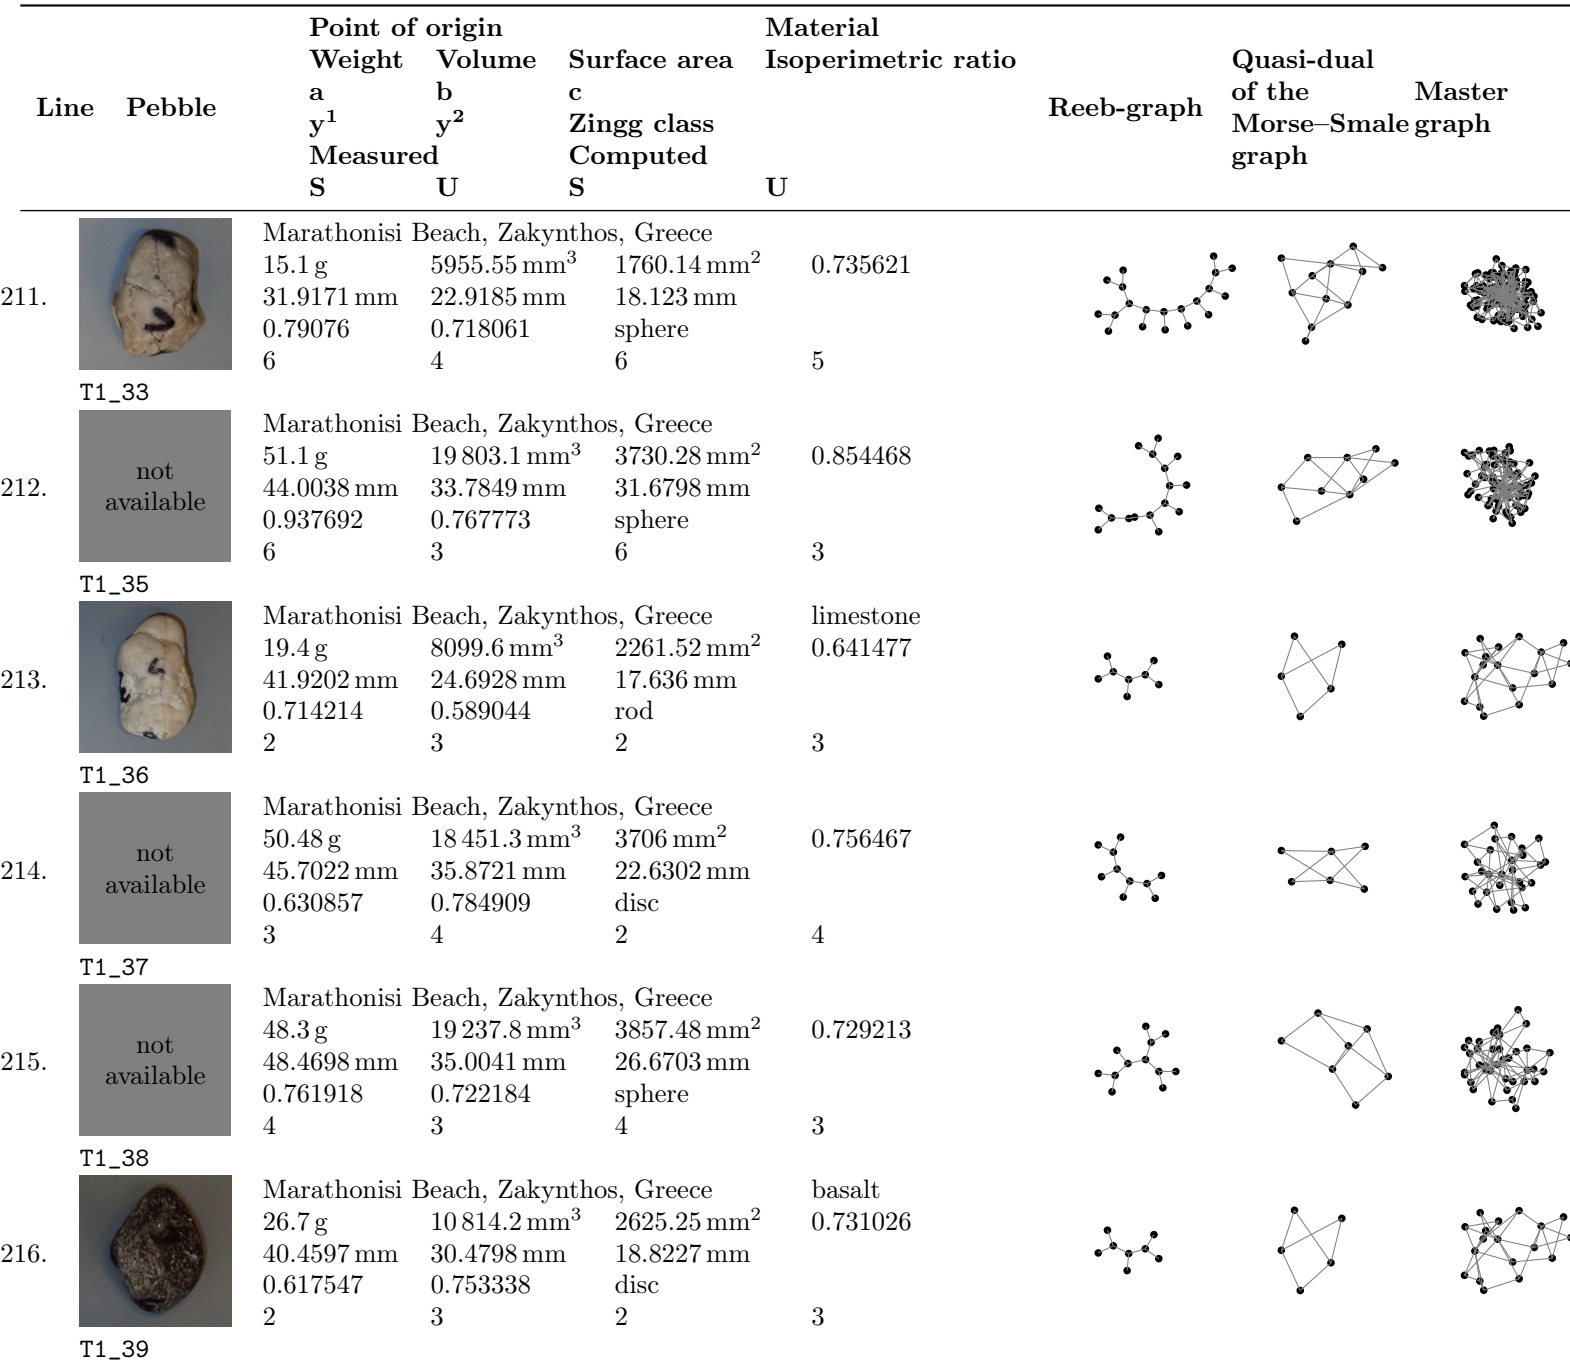 | Marathonisi Beach, Zakynthos, Greece |                          |                         |                     |                                                                                       |                                                                                       |                                                                                       |
|      |                                                                                     | 48.3 g                               | 19 237.8 mm <sup>3</sup> | 3857.48 mm <sup>2</sup> | 0.729213            |                                                                                       |                                                                                       |                                                                                       |
|      |                                                                                     | 48.4698 mm                           | 35.0041 mm               | 26.6703 mm              |                     |                                                                                       |                                                                                       |                                                                                       |
|      |                                                                                     | 0.761918                             | 0.722184                 | sphere                  |                     |                                                                                       |                                                                                       |                                                                                       |
|      |                                                                                     | 4                                    | 3                        | 4                       | 3                   | 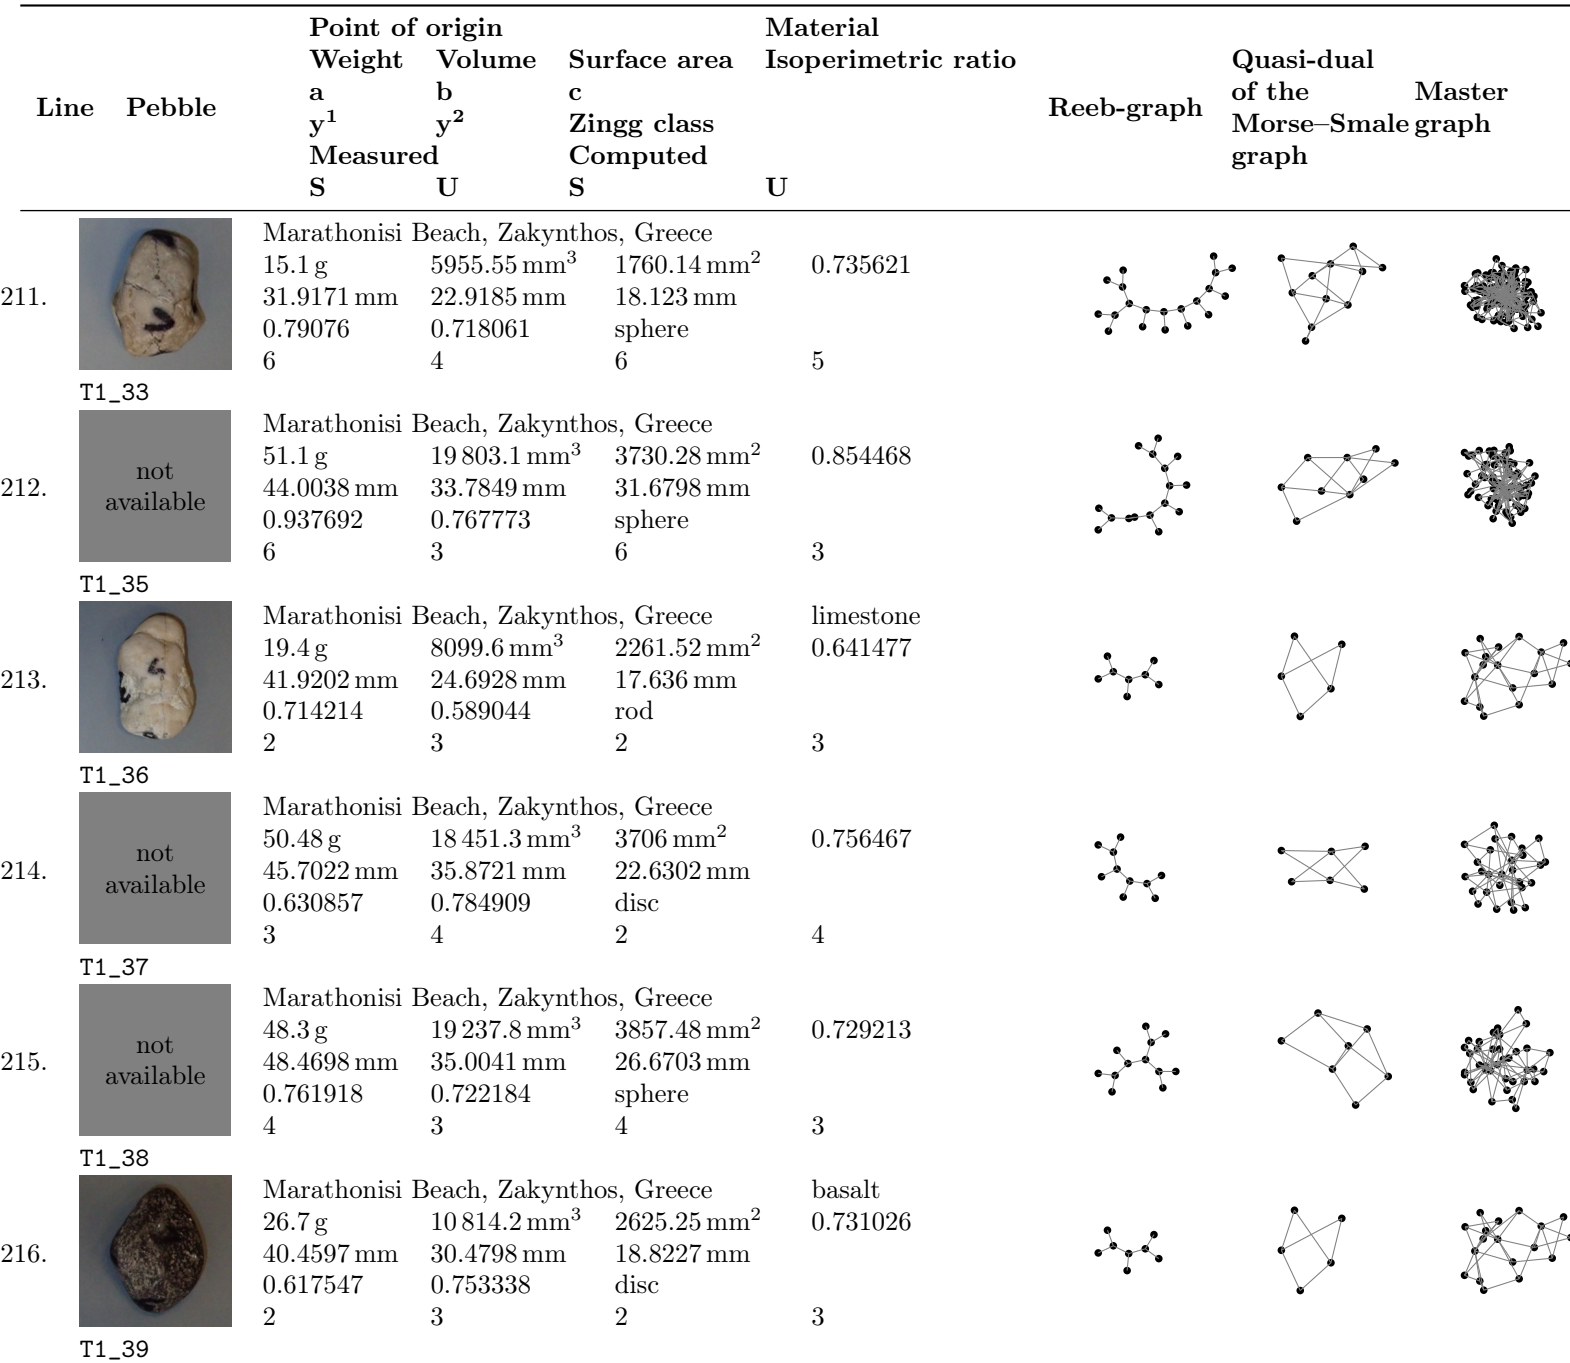 | 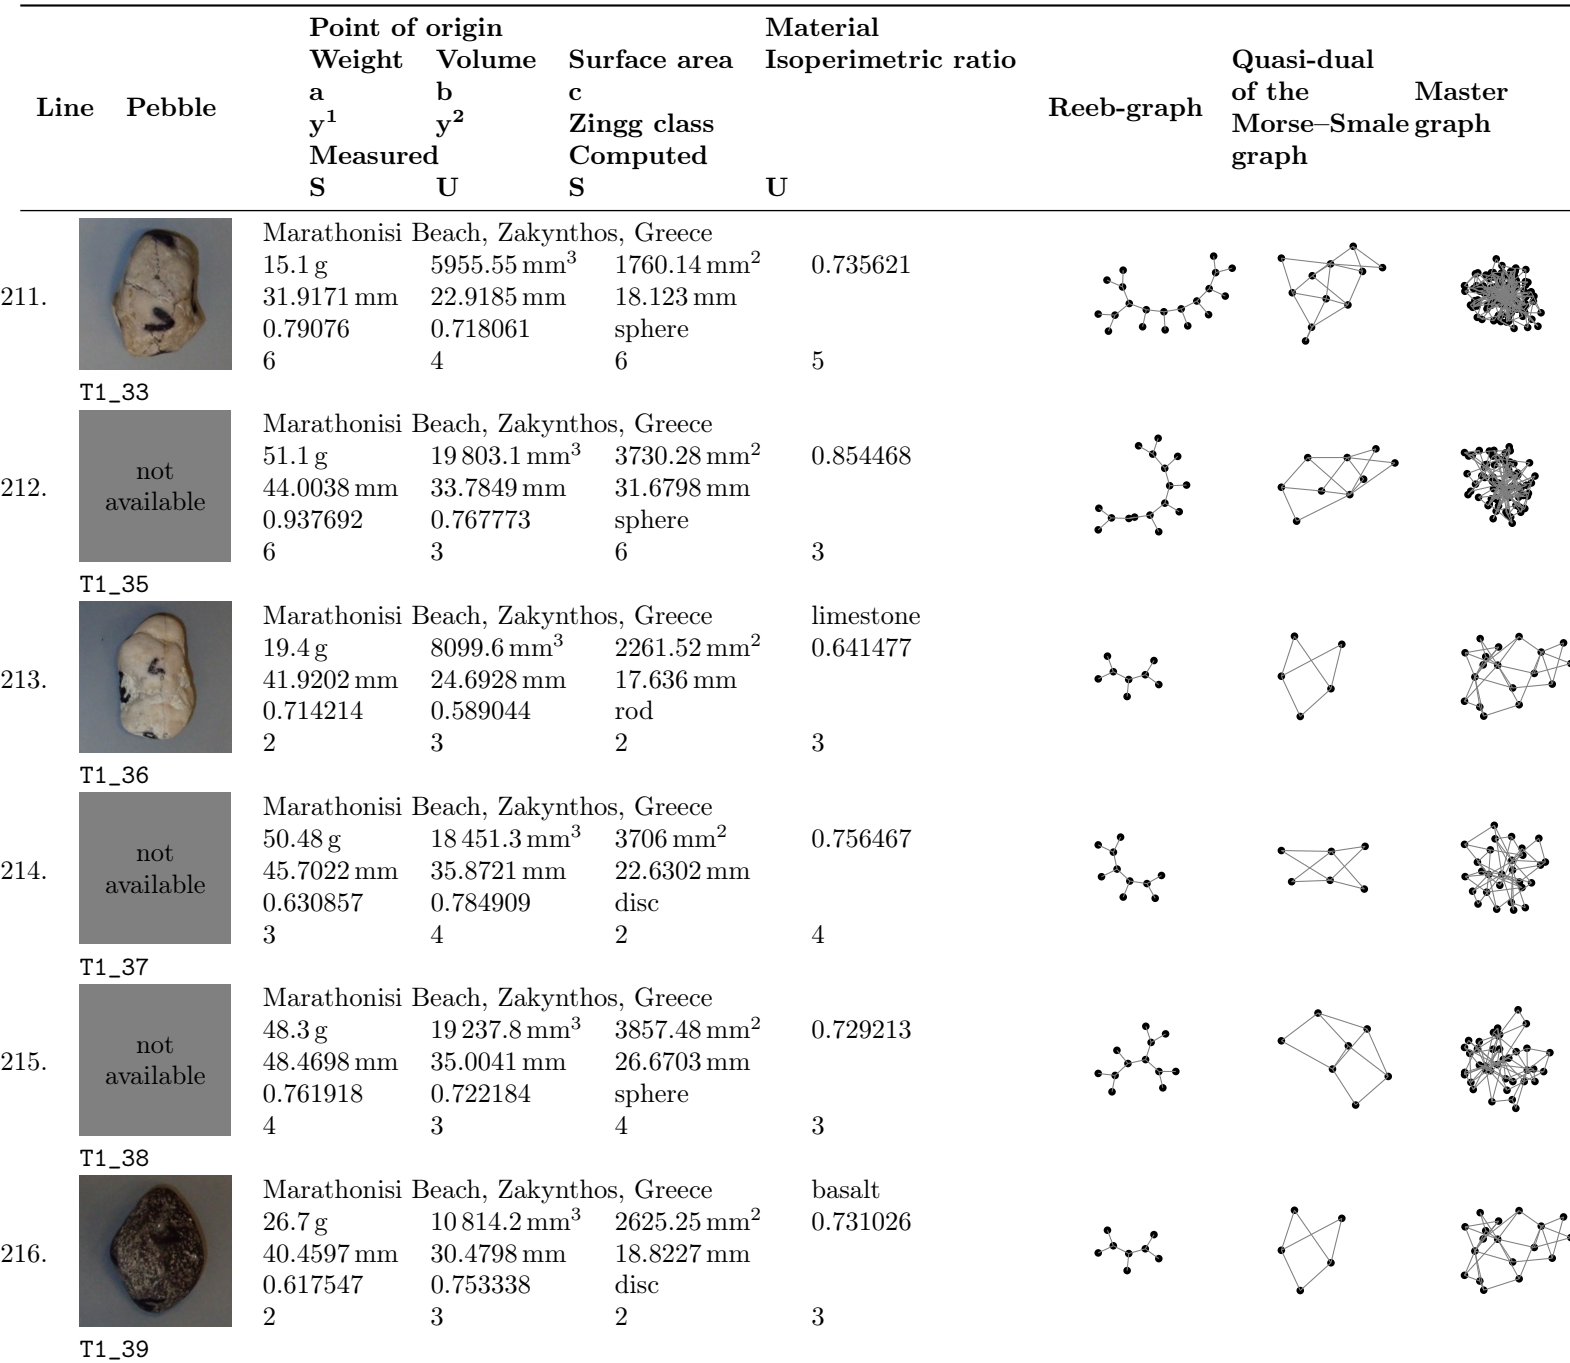 | 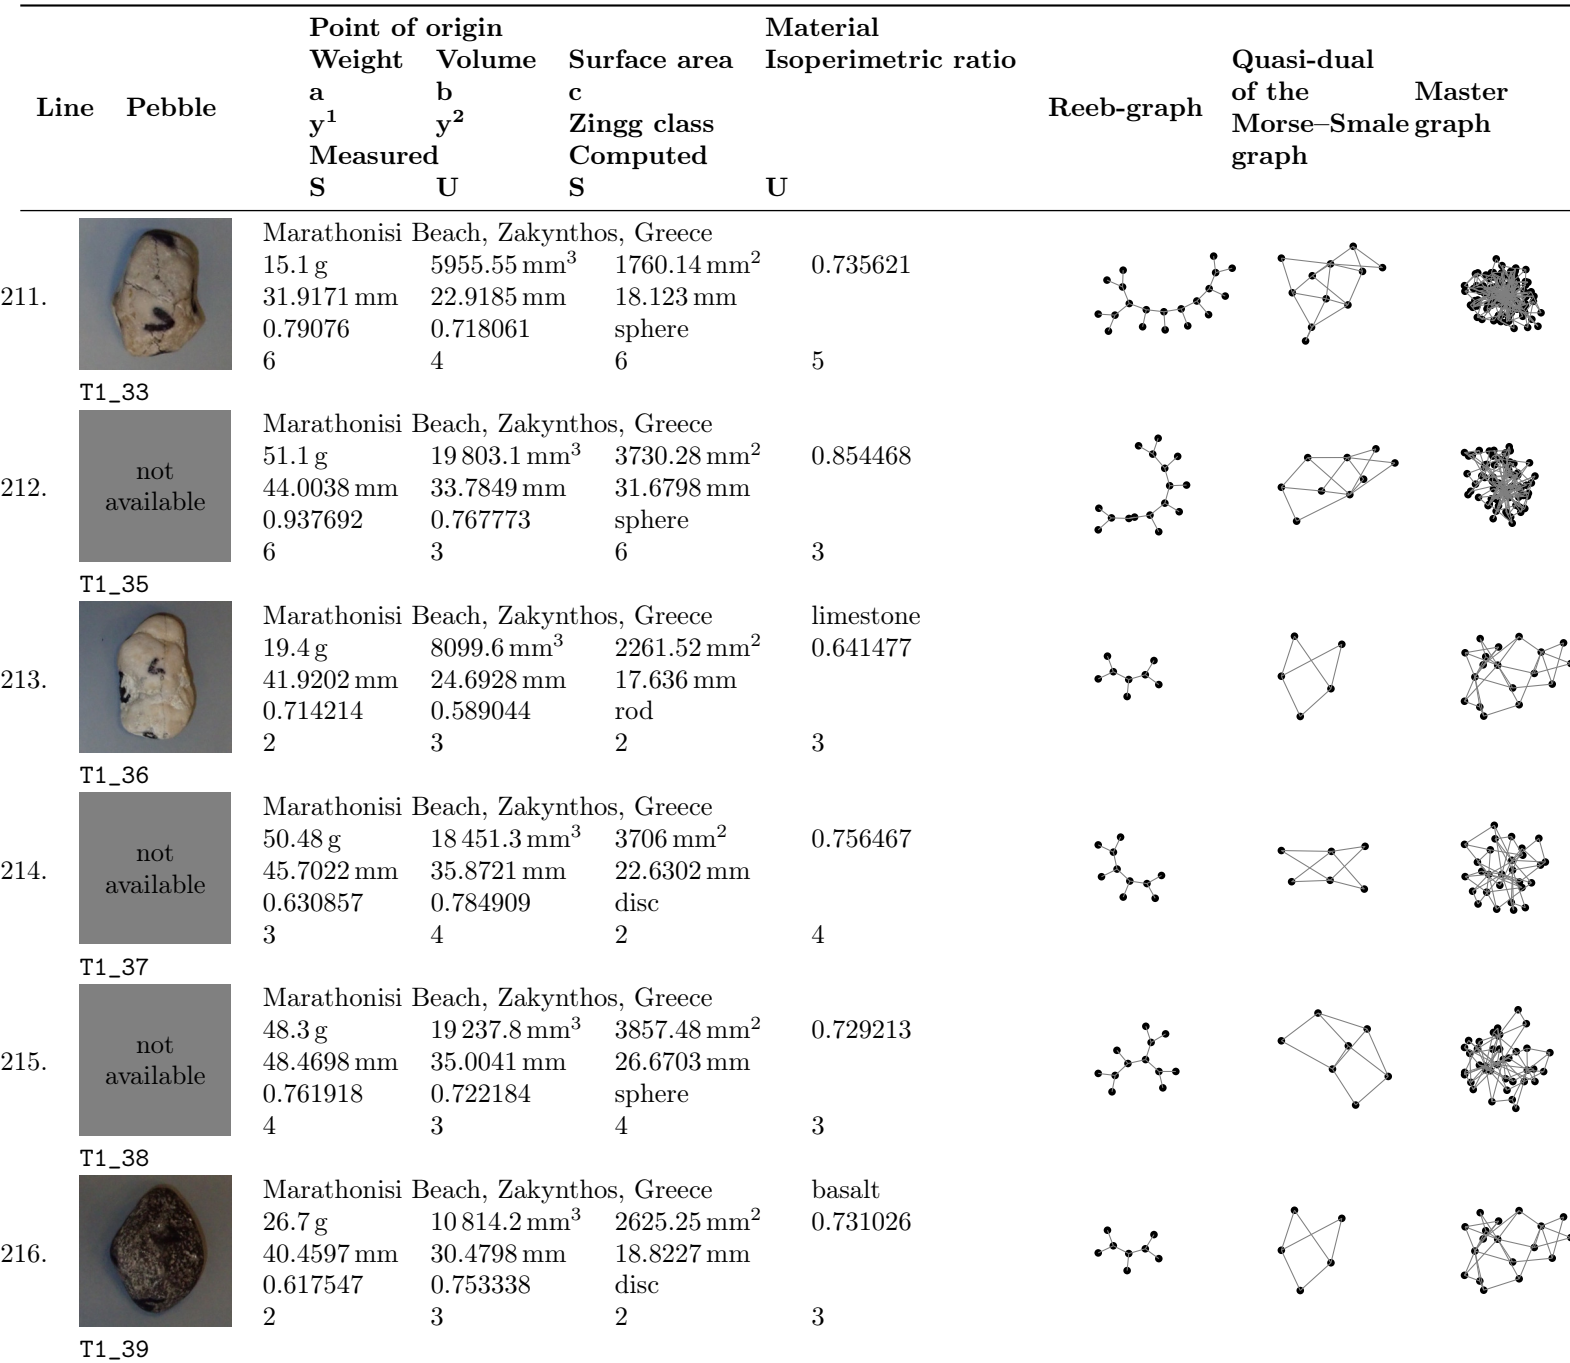 |
|      | T1_38                                                                               |                                      |                          |                         |                     |                                                                                       |                                                                                       |                                                                                       |
| 216. | 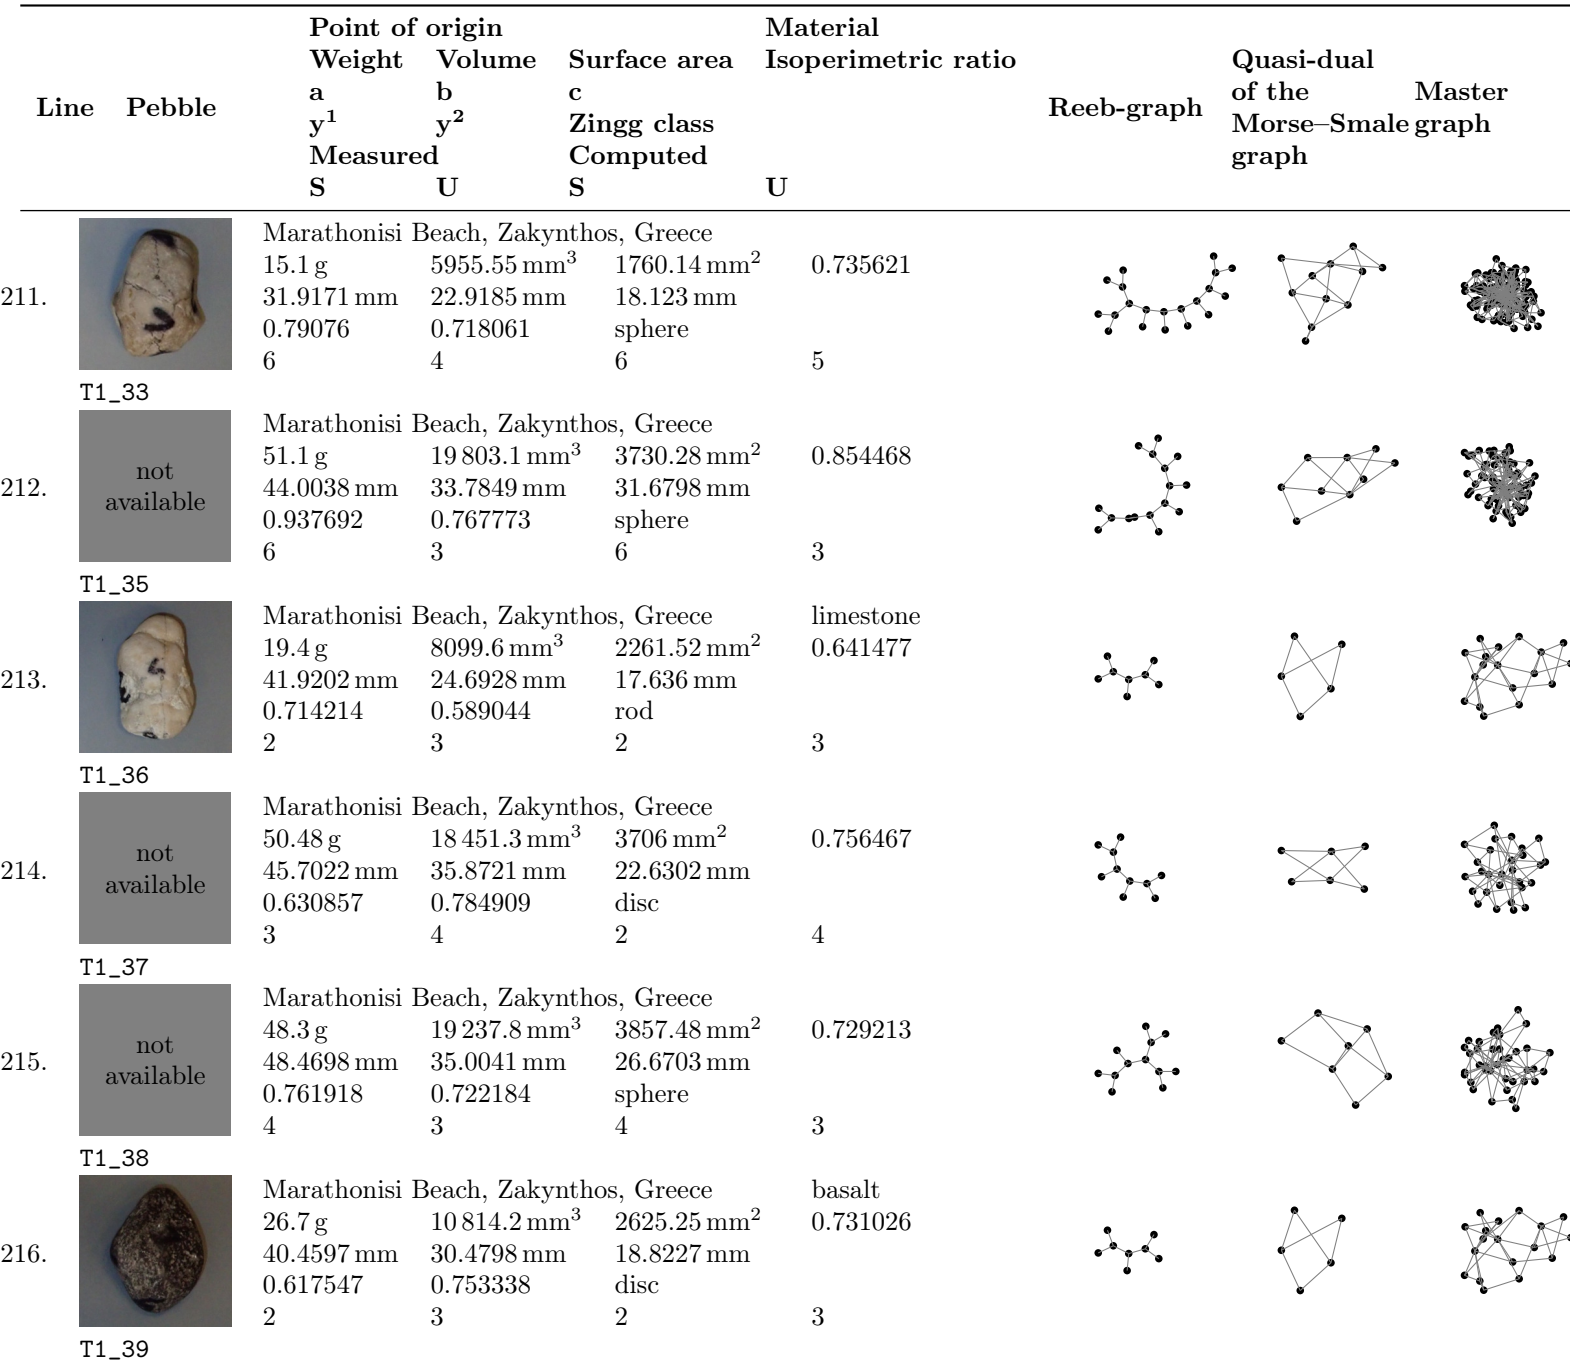 | Marathonisi Beach, Zakynthos, Greece |                          |                         | basalt              |                                                                                       |                                                                                       |                                                                                       |
|      |                                                                                     | 26.7 g                               | 10 814.2 mm <sup>3</sup> | 2625.25 mm <sup>2</sup> | 0.731026            |                                                                                       |                                                                                       |                                                                                       |
|      |                                                                                     | 40.4597 mm                           | 30.4798 mm               | 18.8227 mm              |                     |                                                                                       |                                                                                       |                                                                                       |
|      |                                                                                     | 0.617547                             | 0.753338                 | disc                    |                     |                                                                                       |                                                                                       |                                                                                       |
|      |                                                                                     | 2                                    | 3                        | 2                       | 3                   | 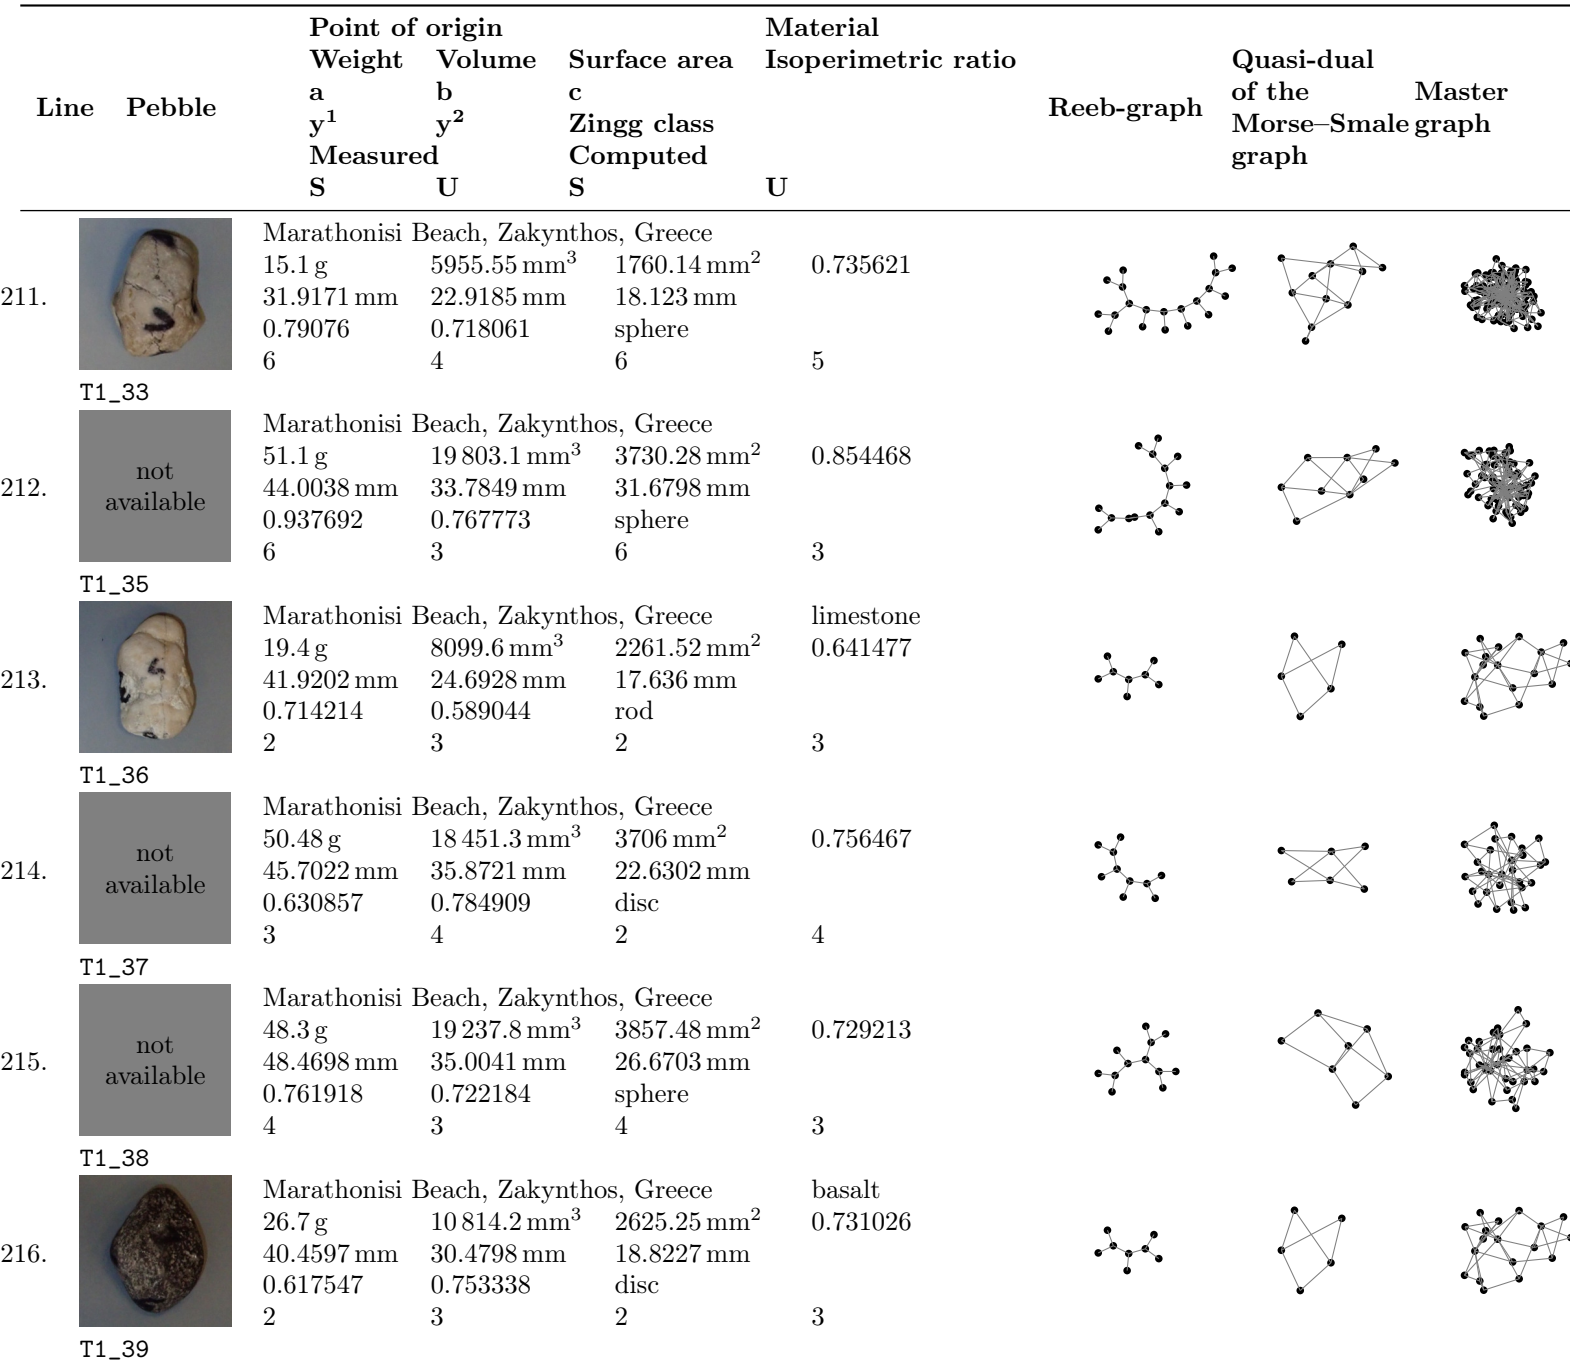 | 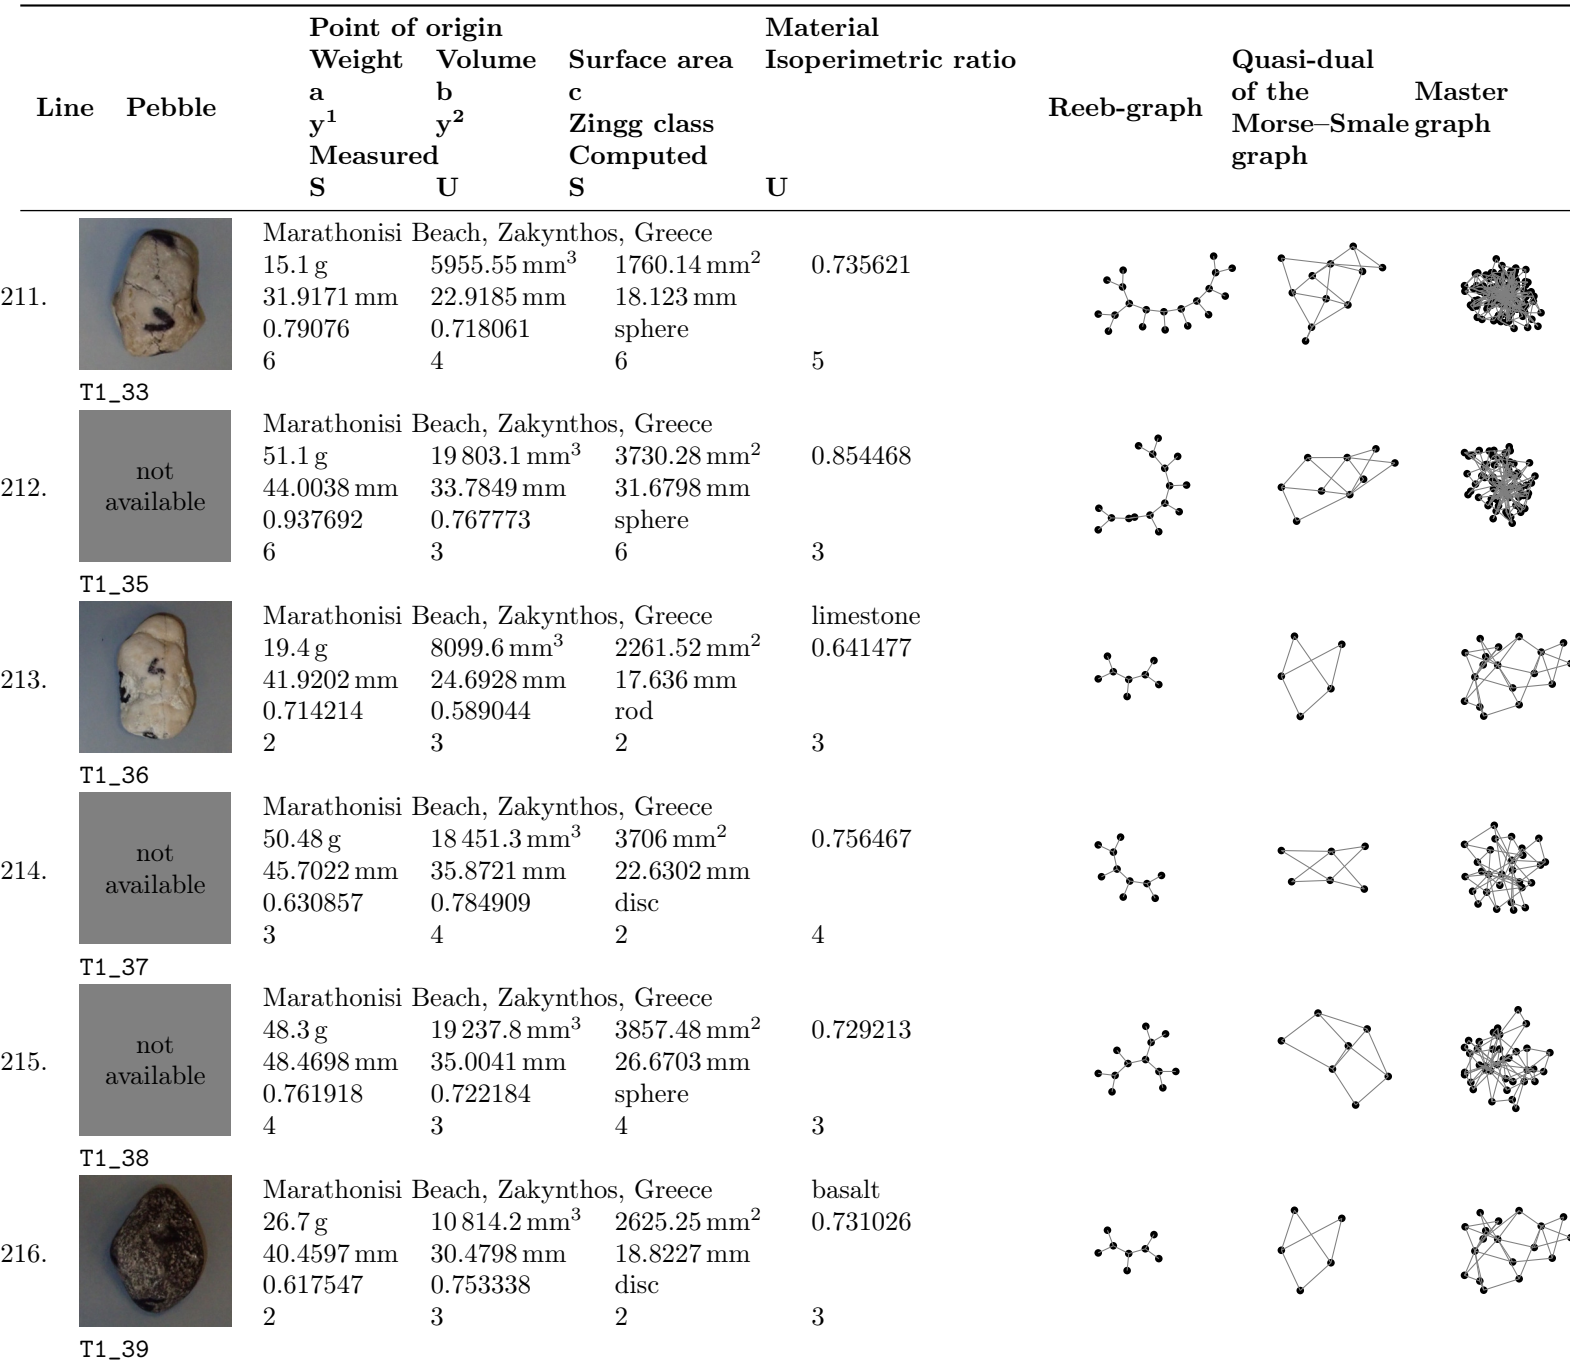 | 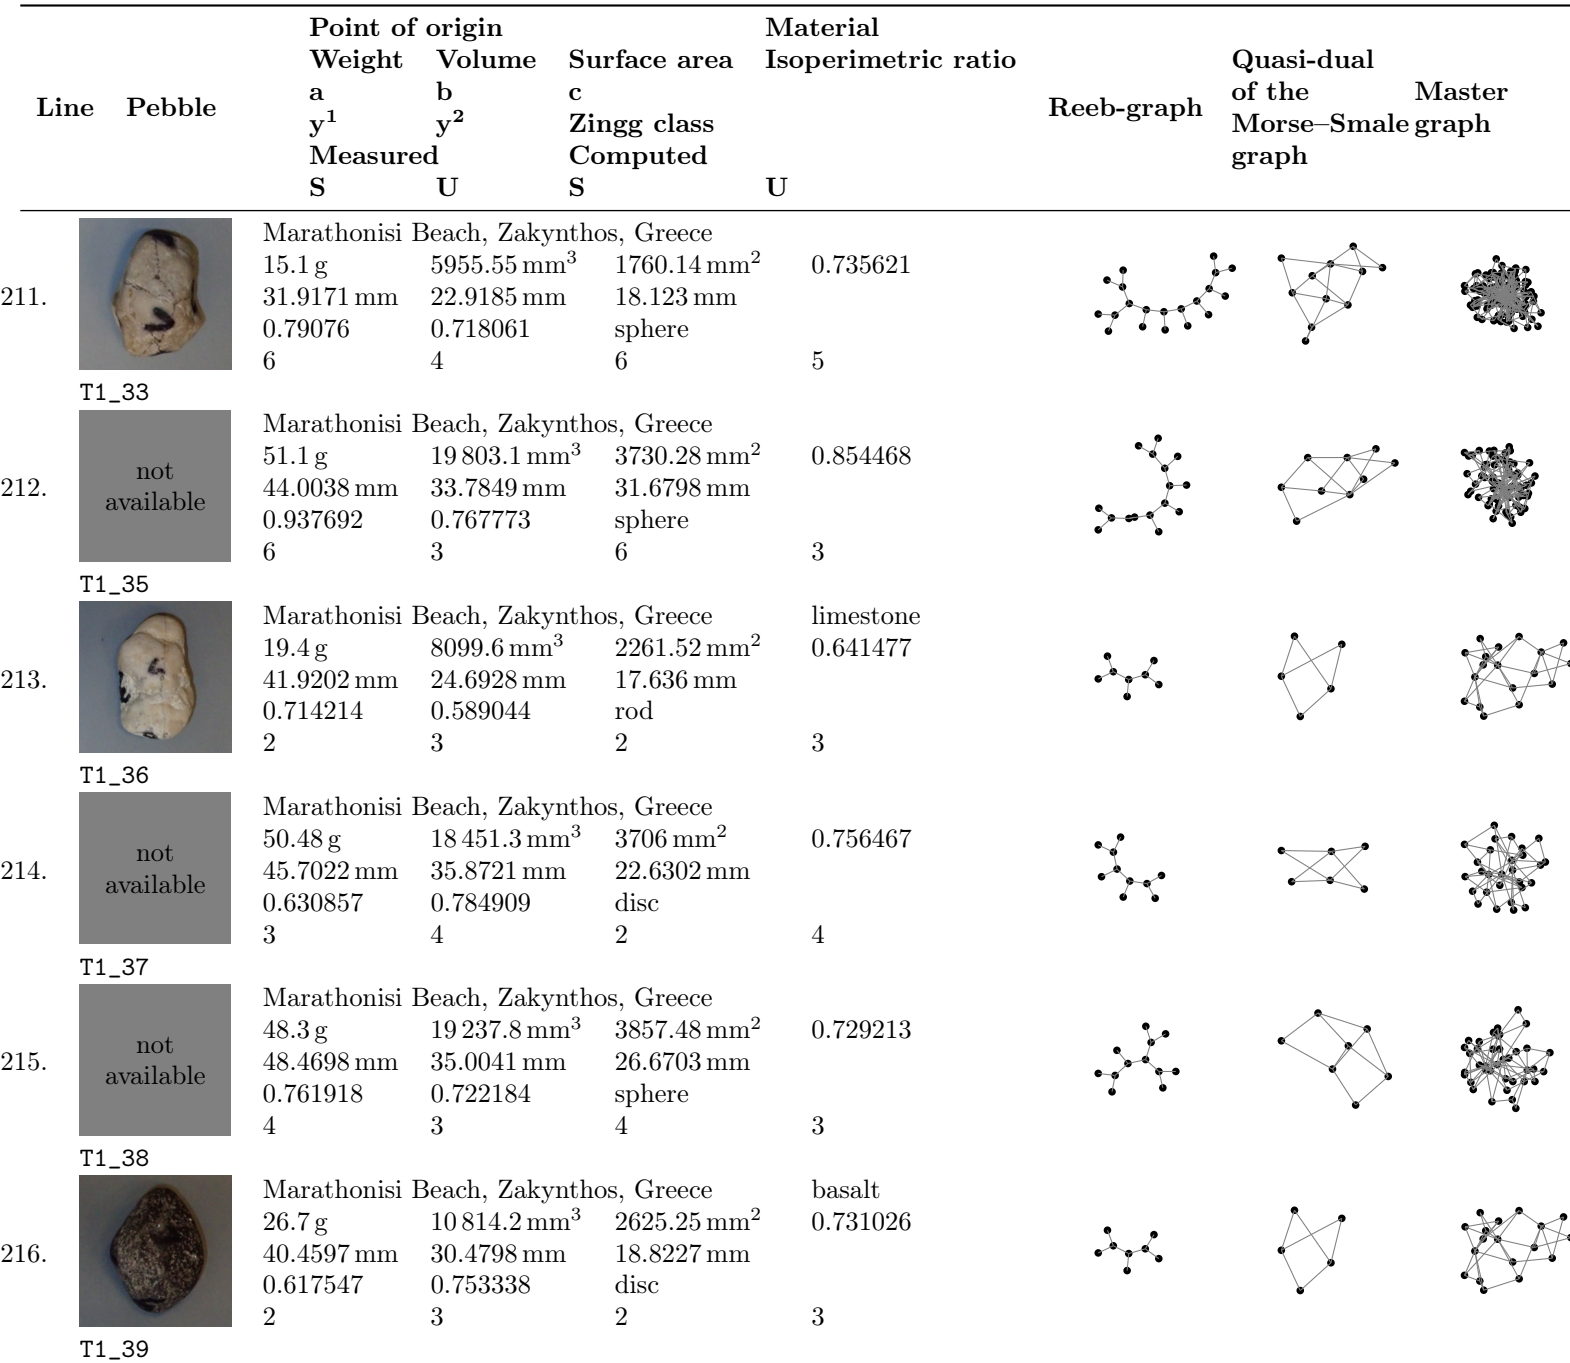 |
|      | T1_39                                                                               |                                      |                          |                         |                     |                                                                                       |                                                                                       |                                                                                       |

| Line | Pebble                                                                              | Point of origin                                                                |                                                         | Surface area<br>c<br>Zingg class<br>Computed<br>S    | Material<br>Isoperimetric ratio<br>U | Reeb-graph                                                                            | Quasi-dual<br>of the<br>Morse–Smale<br>graph                                          | Master<br>graph                                                                       |
|------|-------------------------------------------------------------------------------------|--------------------------------------------------------------------------------|---------------------------------------------------------|------------------------------------------------------|--------------------------------------|---------------------------------------------------------------------------------------|---------------------------------------------------------------------------------------|---------------------------------------------------------------------------------------|
|      |                                                                                     | Weight                                                                         | Volume                                                  |                                                      |                                      |                                                                                       |                                                                                       |                                                                                       |
|      |                                                                                     | a<br>y <sup>1</sup><br>Measured<br>S                                           | b<br>y <sup>2</sup><br>U                                |                                                      |                                      |                                                                                       |                                                                                       |                                                                                       |
|      |                                                                                     |                                                                                |                                                         |                                                      |                                      |                                                                                       |                                                                                       |                                                                                       |
| 217. | 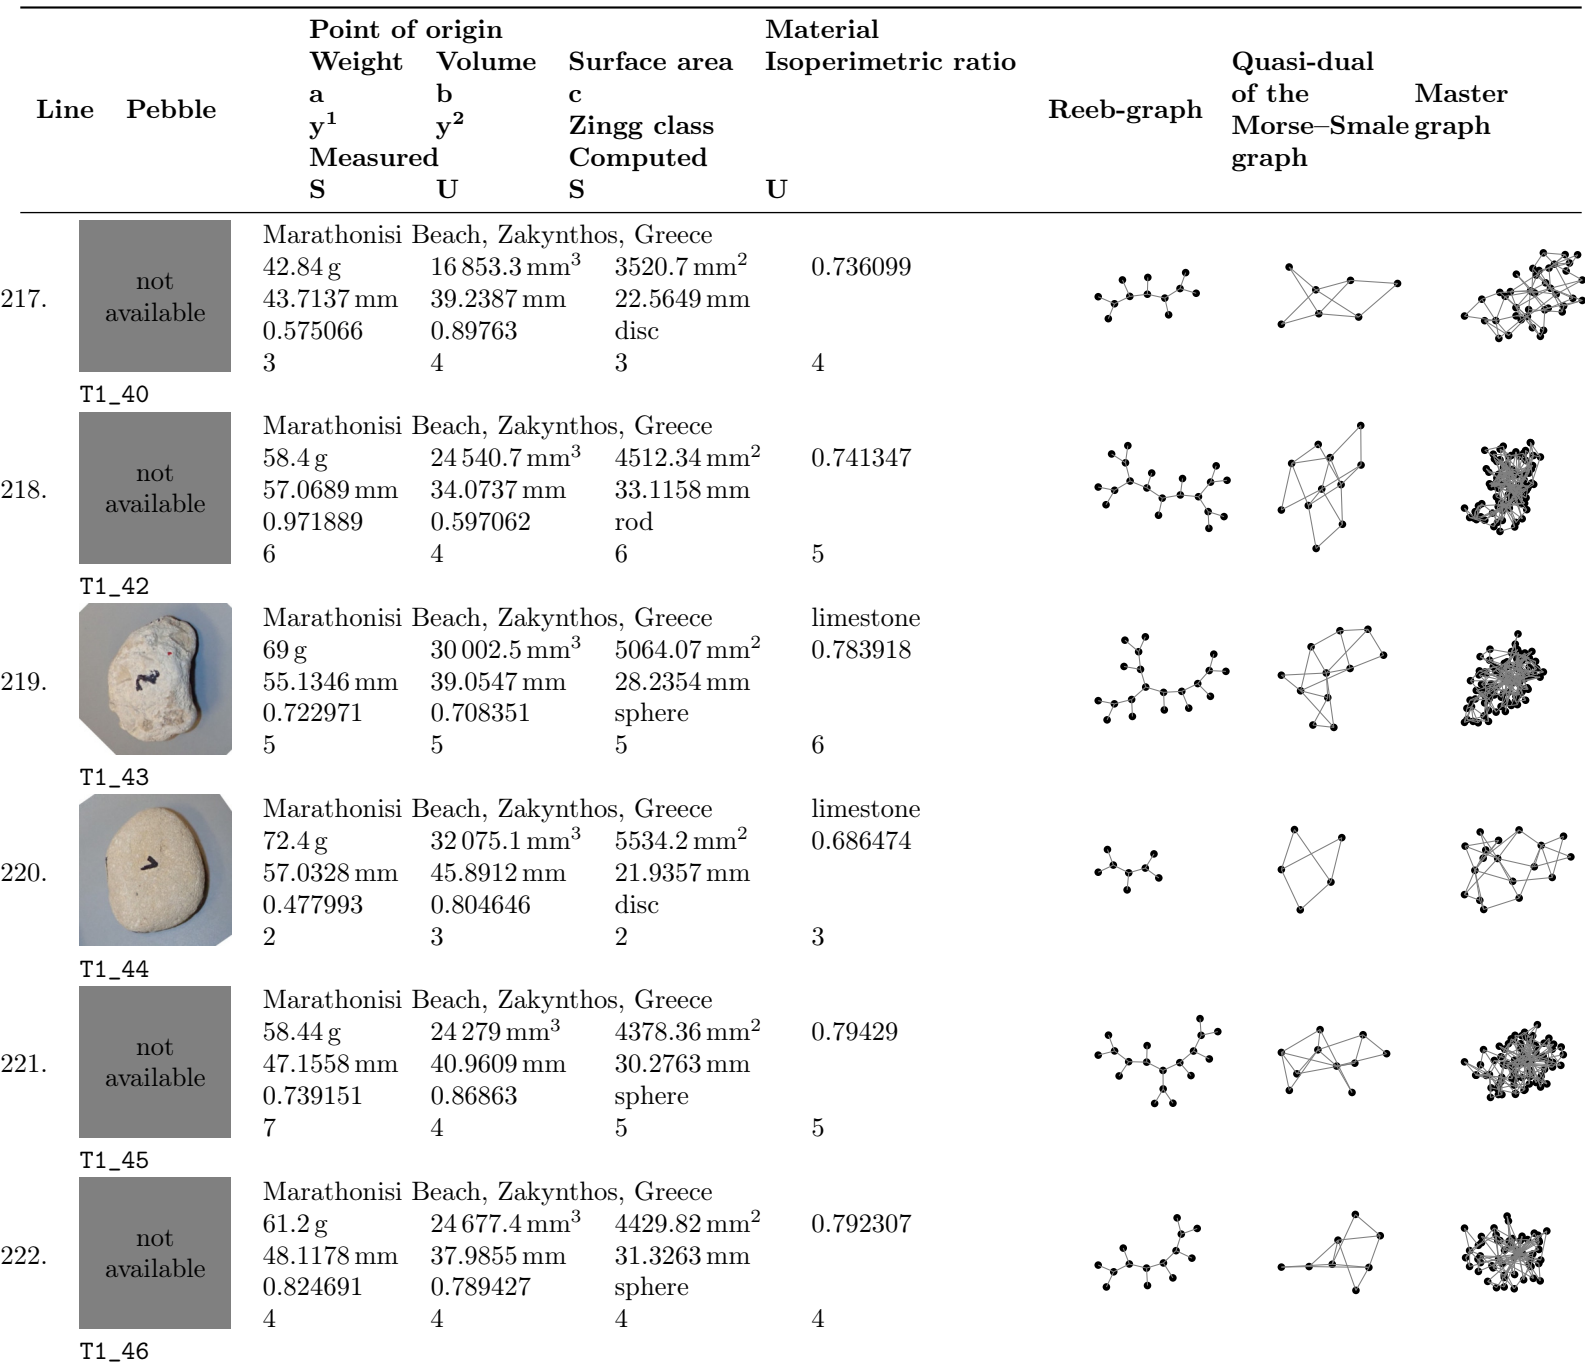   | Marathonisi Beach, Zakynthos, Greece<br>42.84 g<br>43.7137 mm<br>0.575066<br>3 | 16 853.3 mm <sup>3</sup><br>39.2387 mm<br>0.89763<br>4  | 3520.7 mm <sup>2</sup><br>22.5649 mm<br>disc<br>3    | 0.736099<br><br><br>4                | 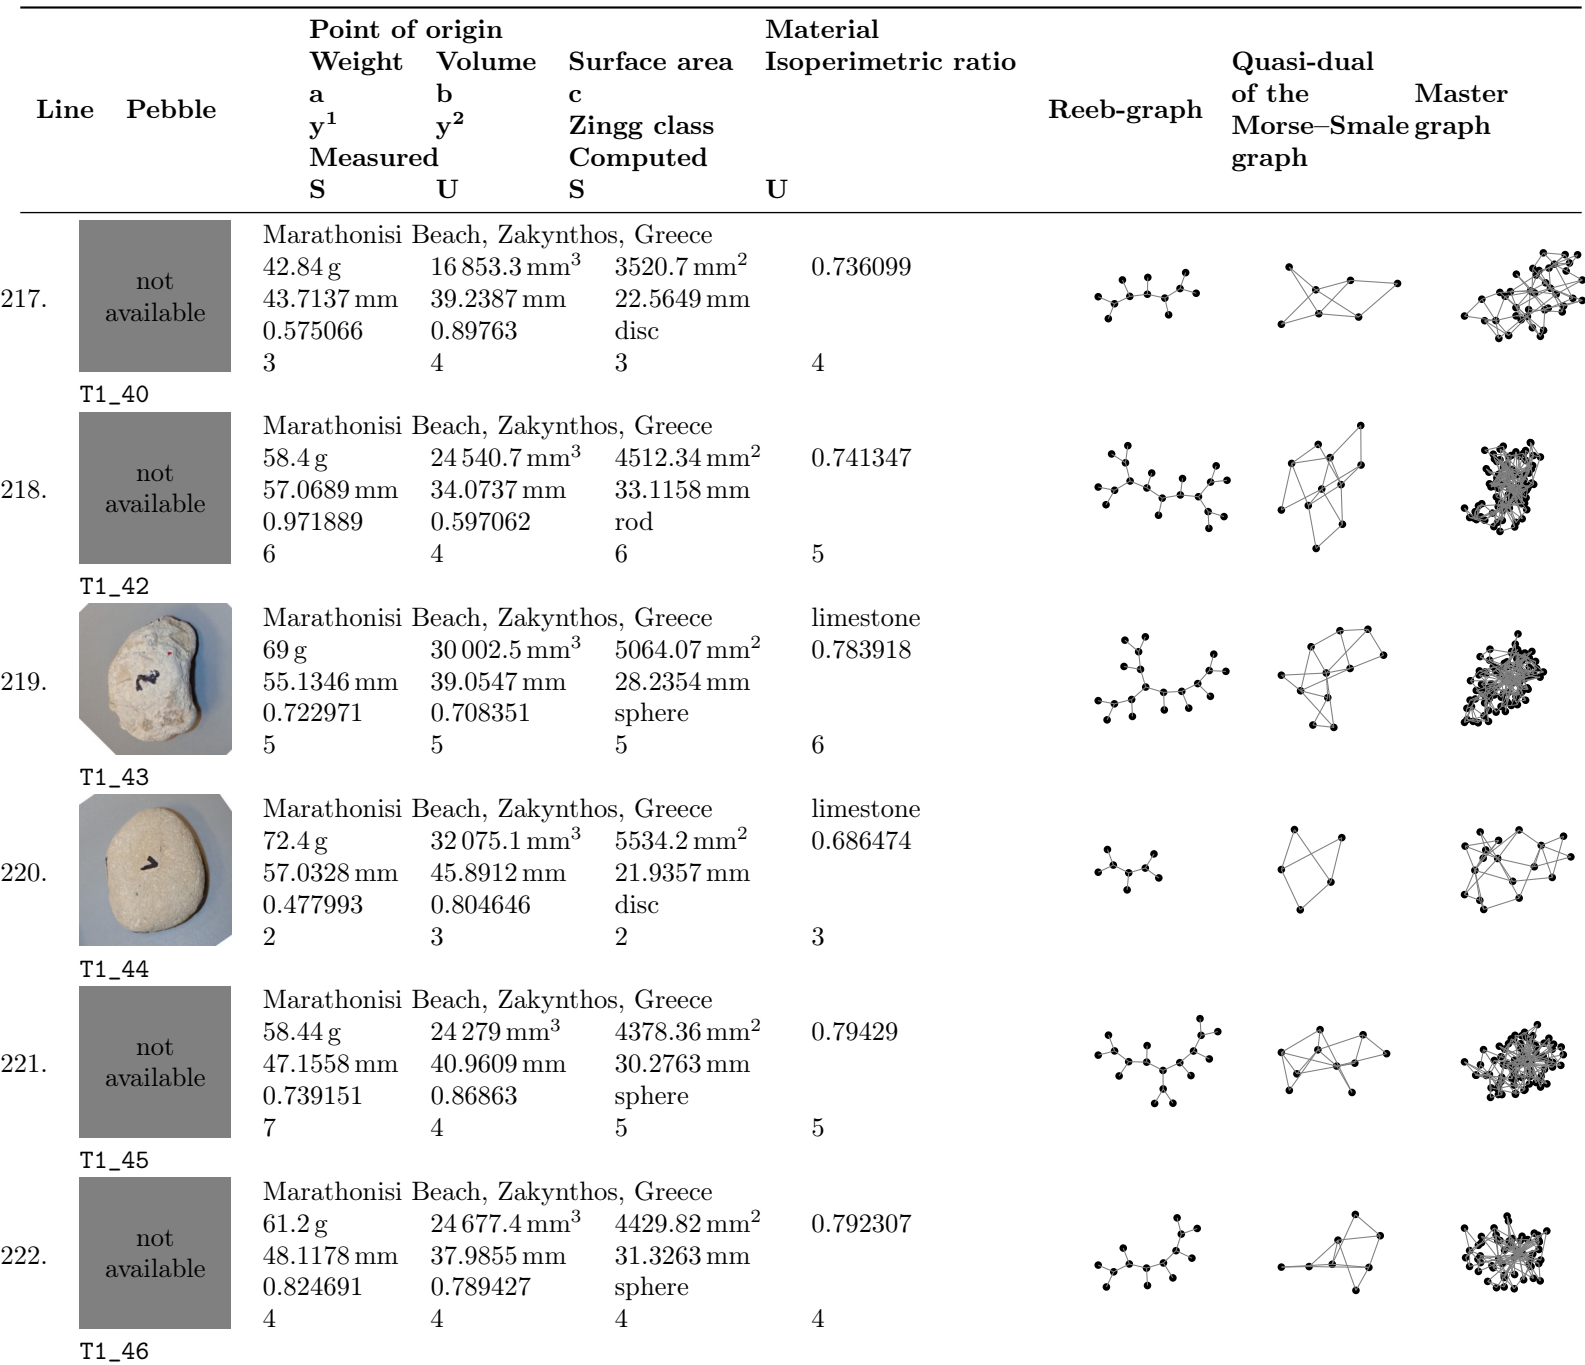   | 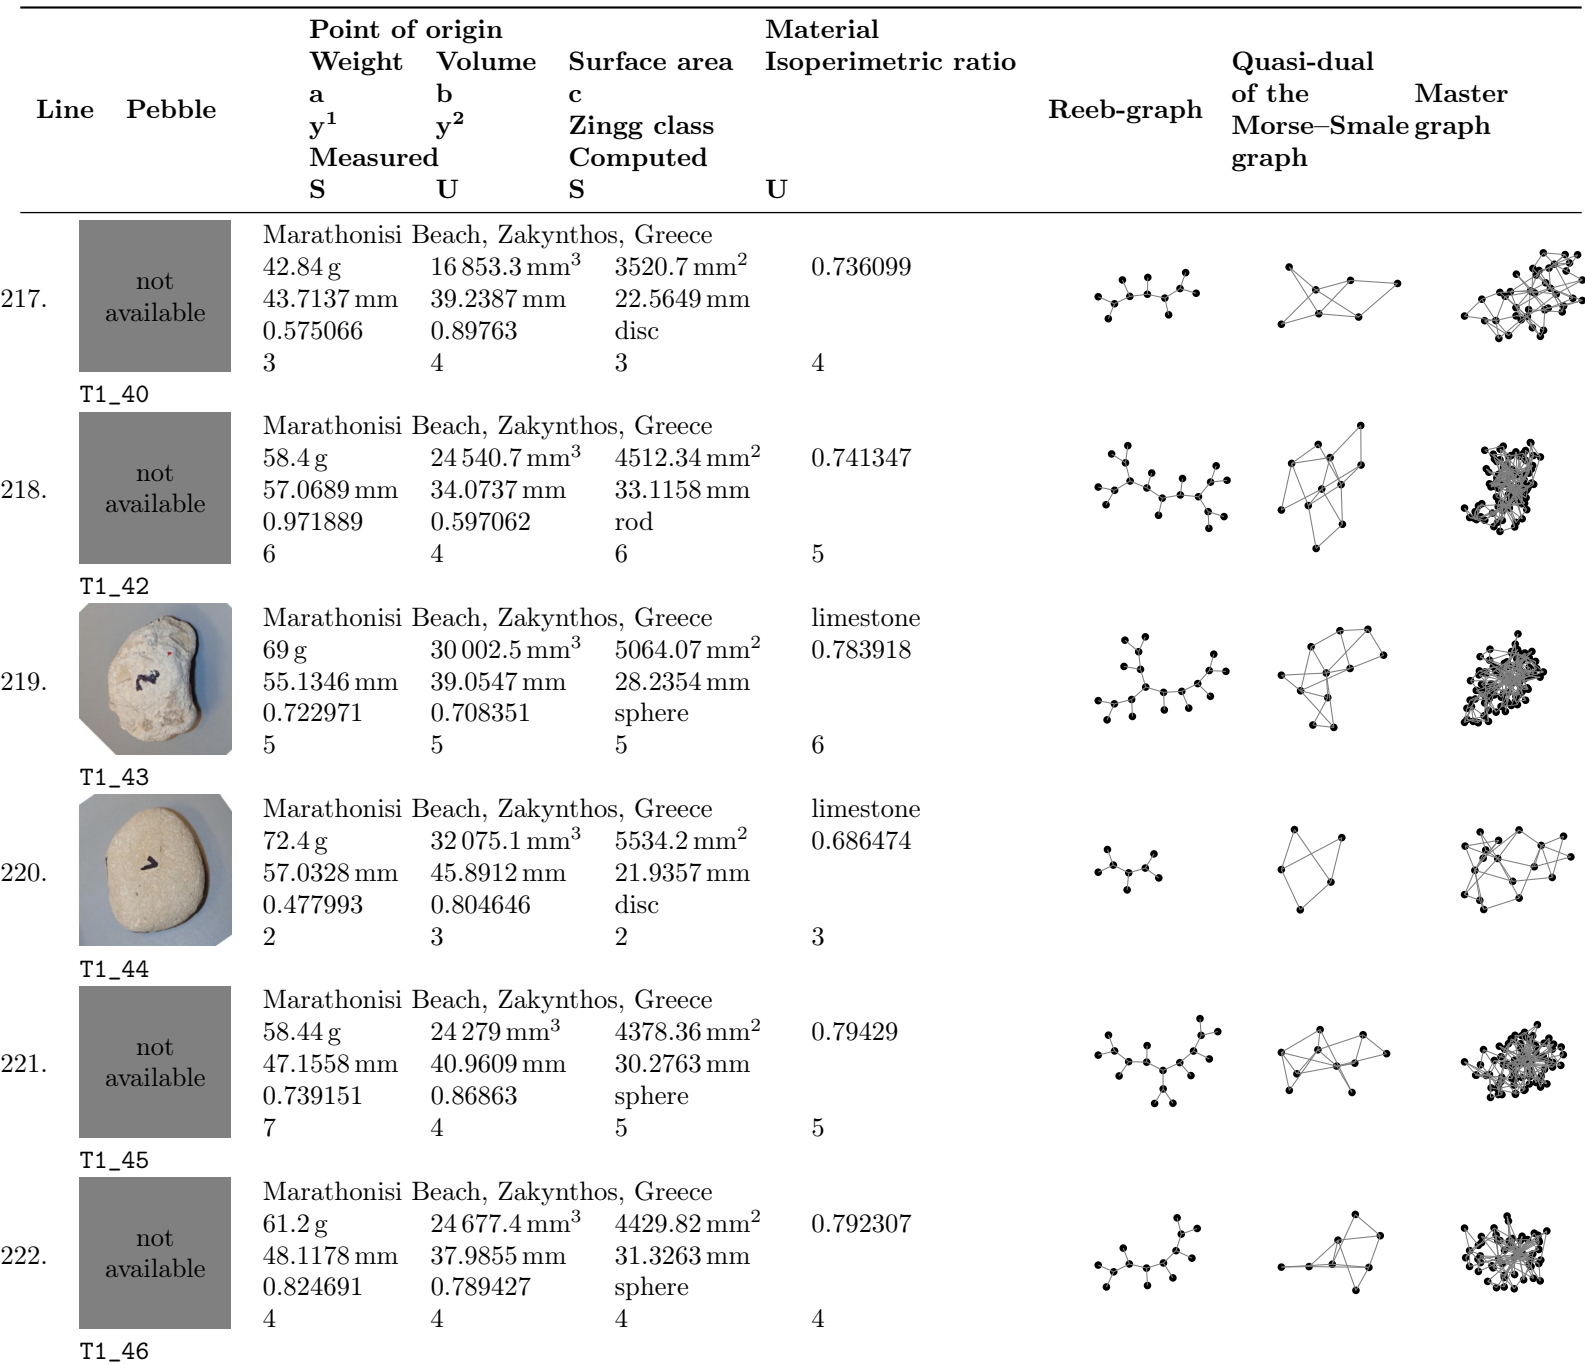   | 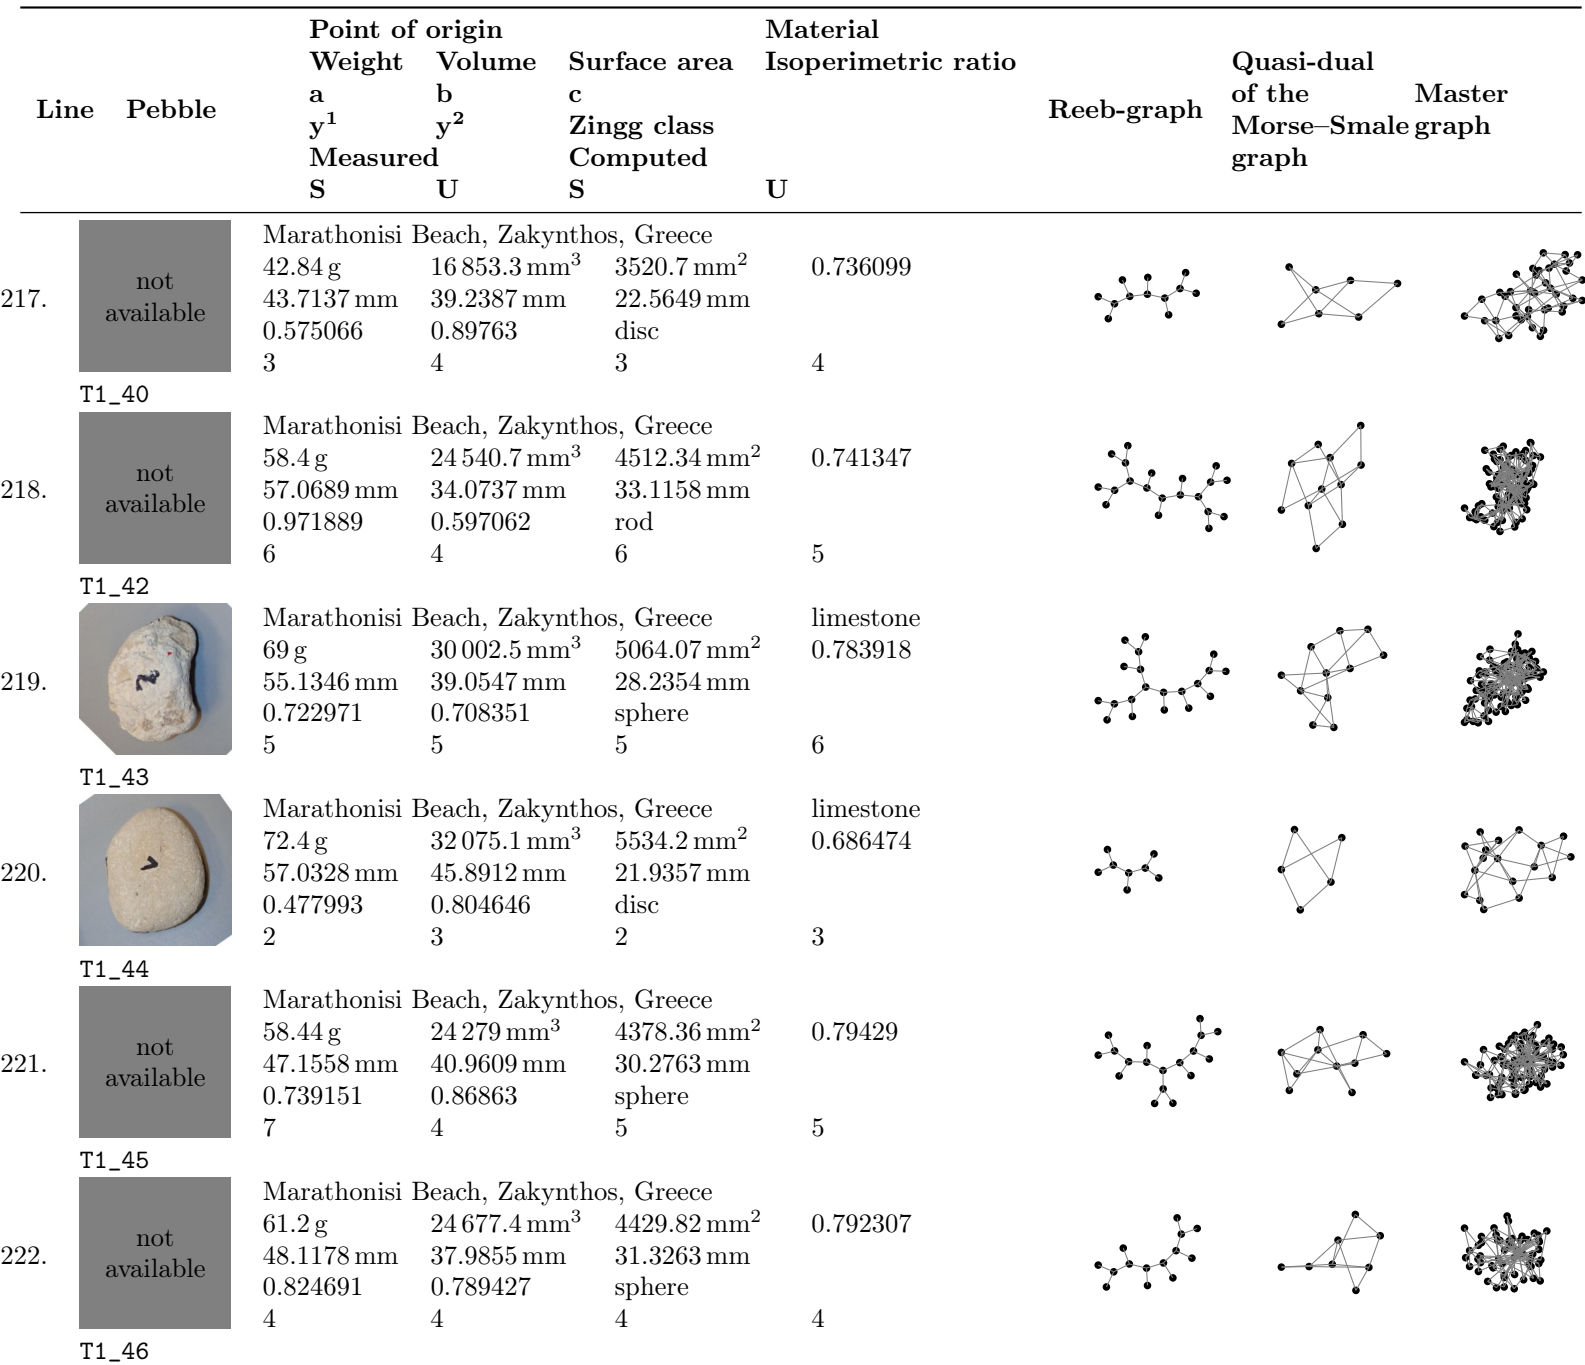   |
|      | T1_40                                                                               |                                                                                |                                                         |                                                      |                                      |                                                                                       |                                                                                       |                                                                                       |
| 218. | 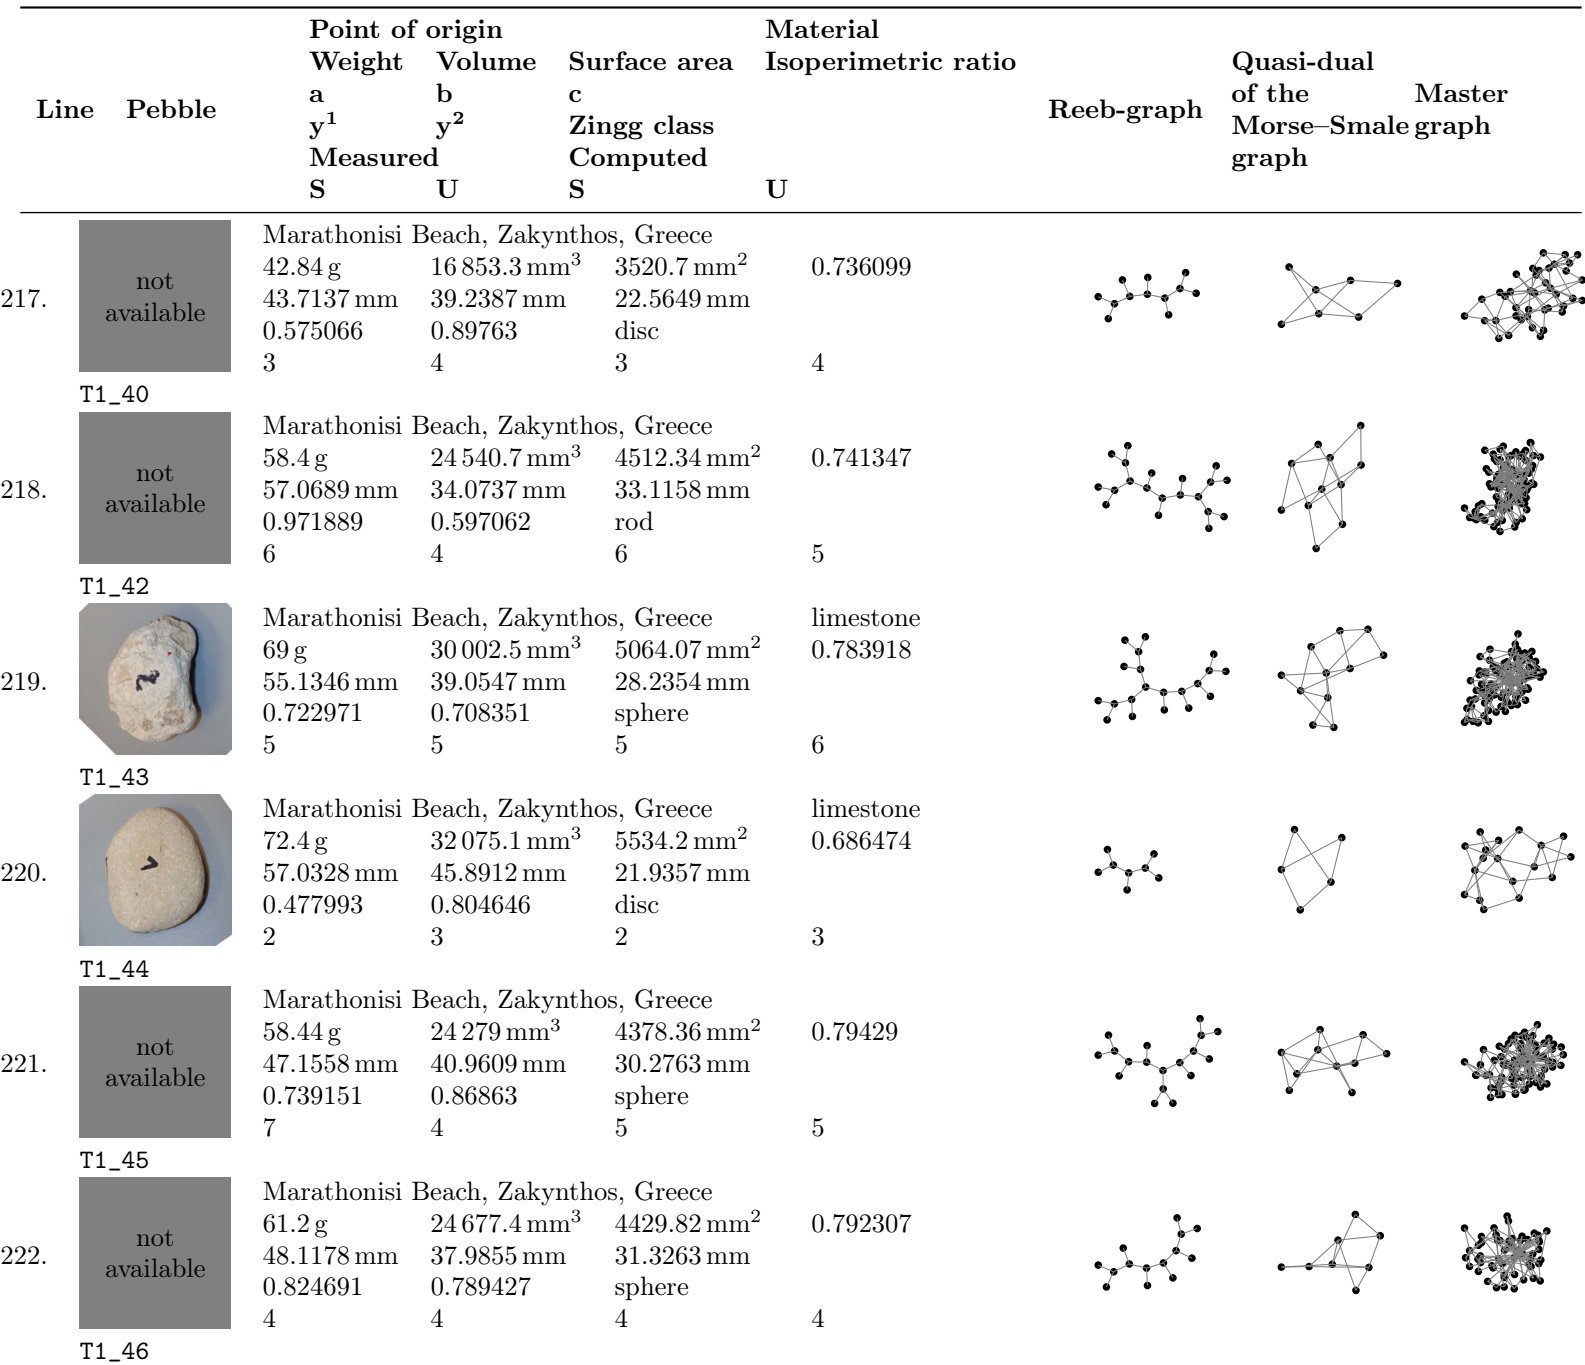   | Marathonisi Beach, Zakynthos, Greece<br>58.4 g<br>57.0689 mm<br>0.971889<br>6  | 24 540.7 mm <sup>3</sup><br>34.0737 mm<br>0.597062<br>4 | 4512.34 mm <sup>2</sup><br>33.1158 mm<br>rod<br>6    | 0.741347<br><br><br>5                | 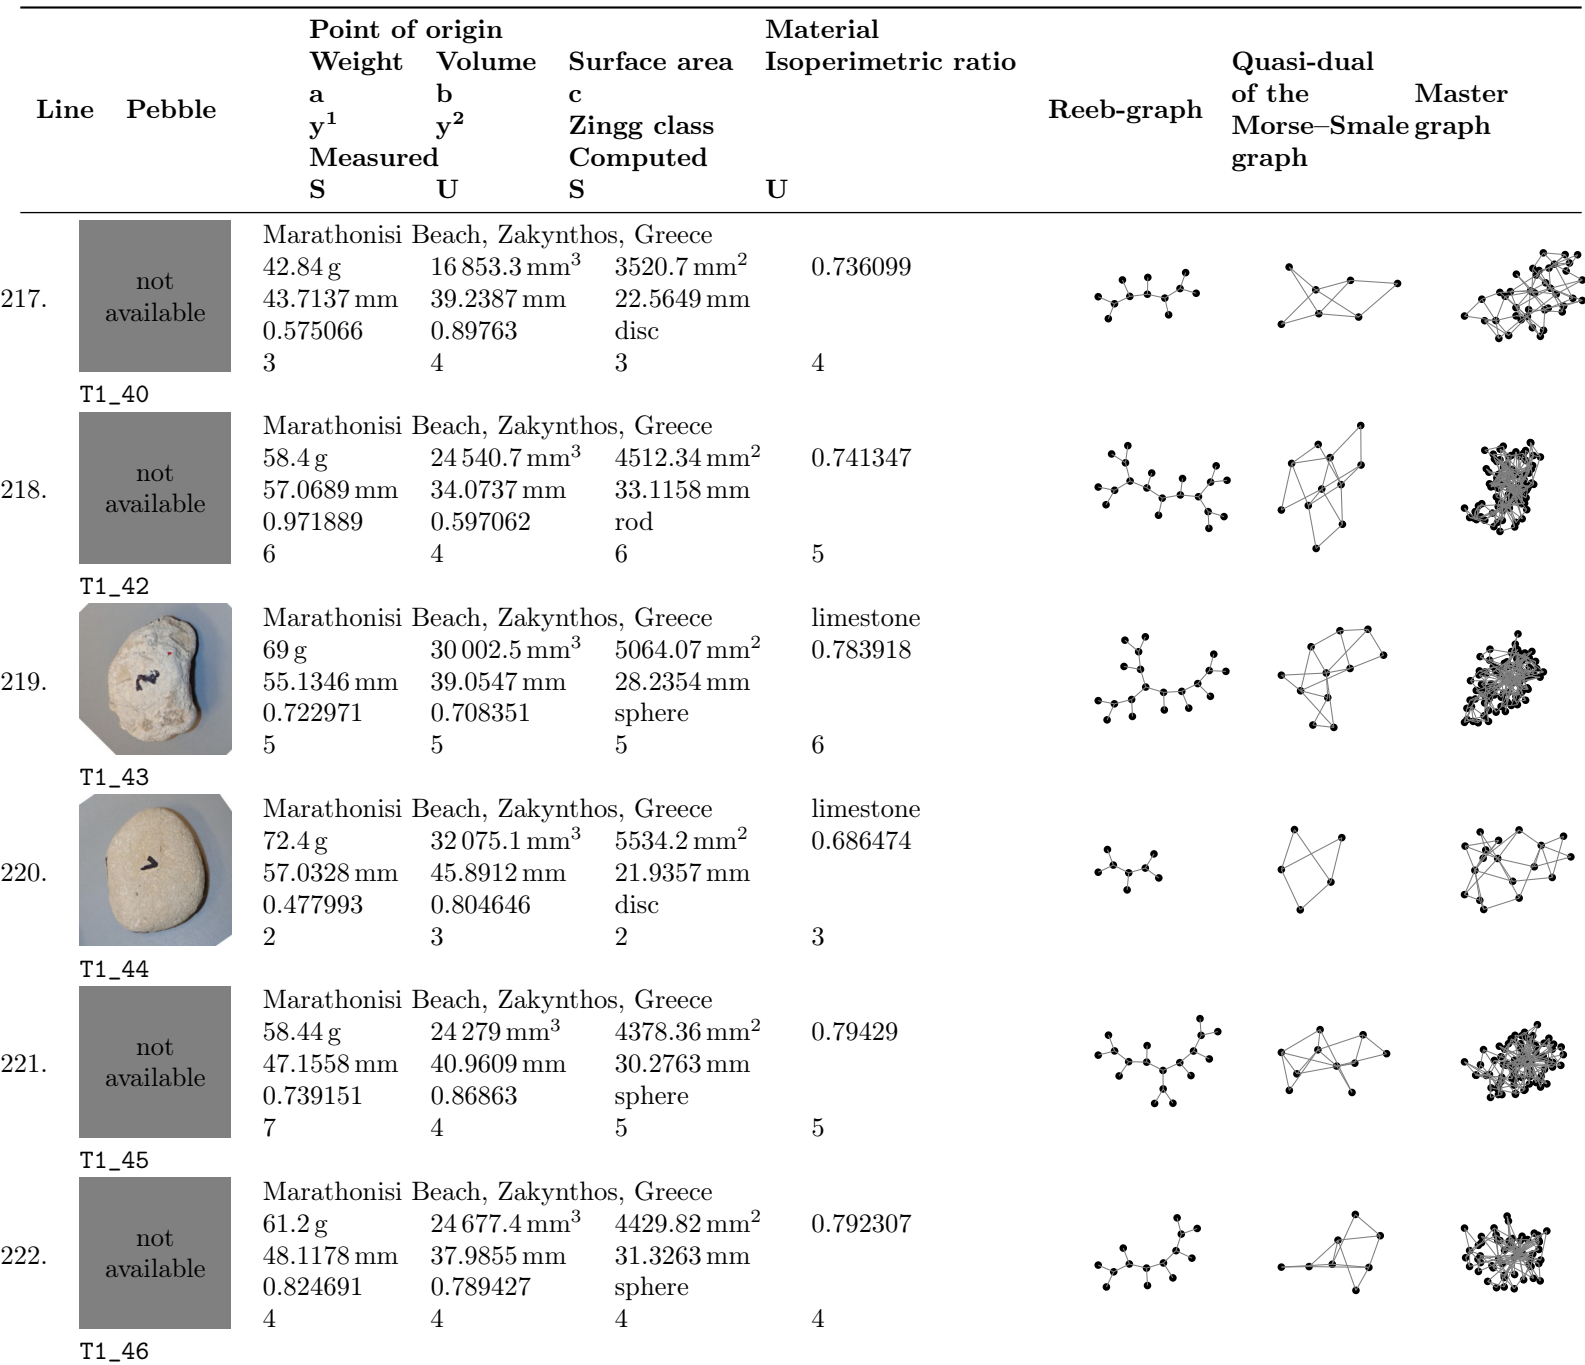   | 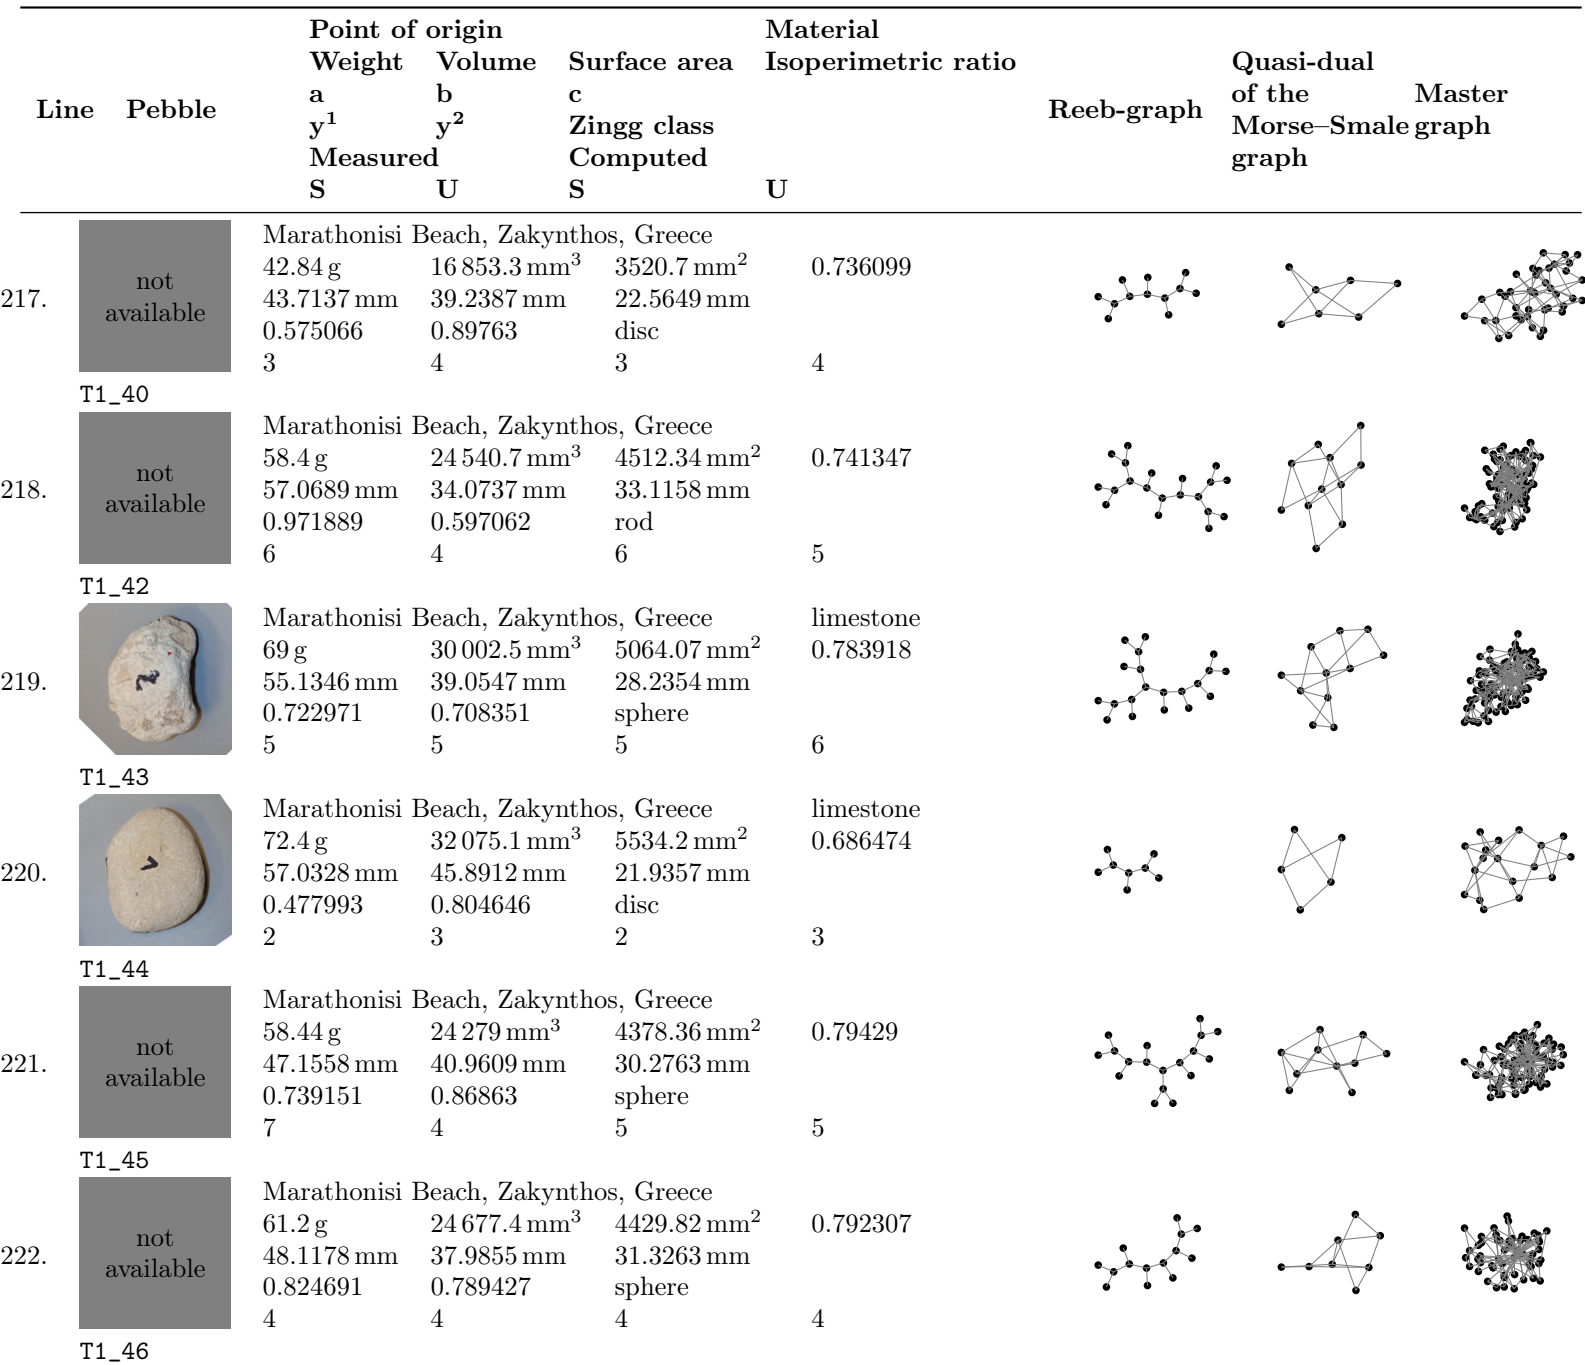   | 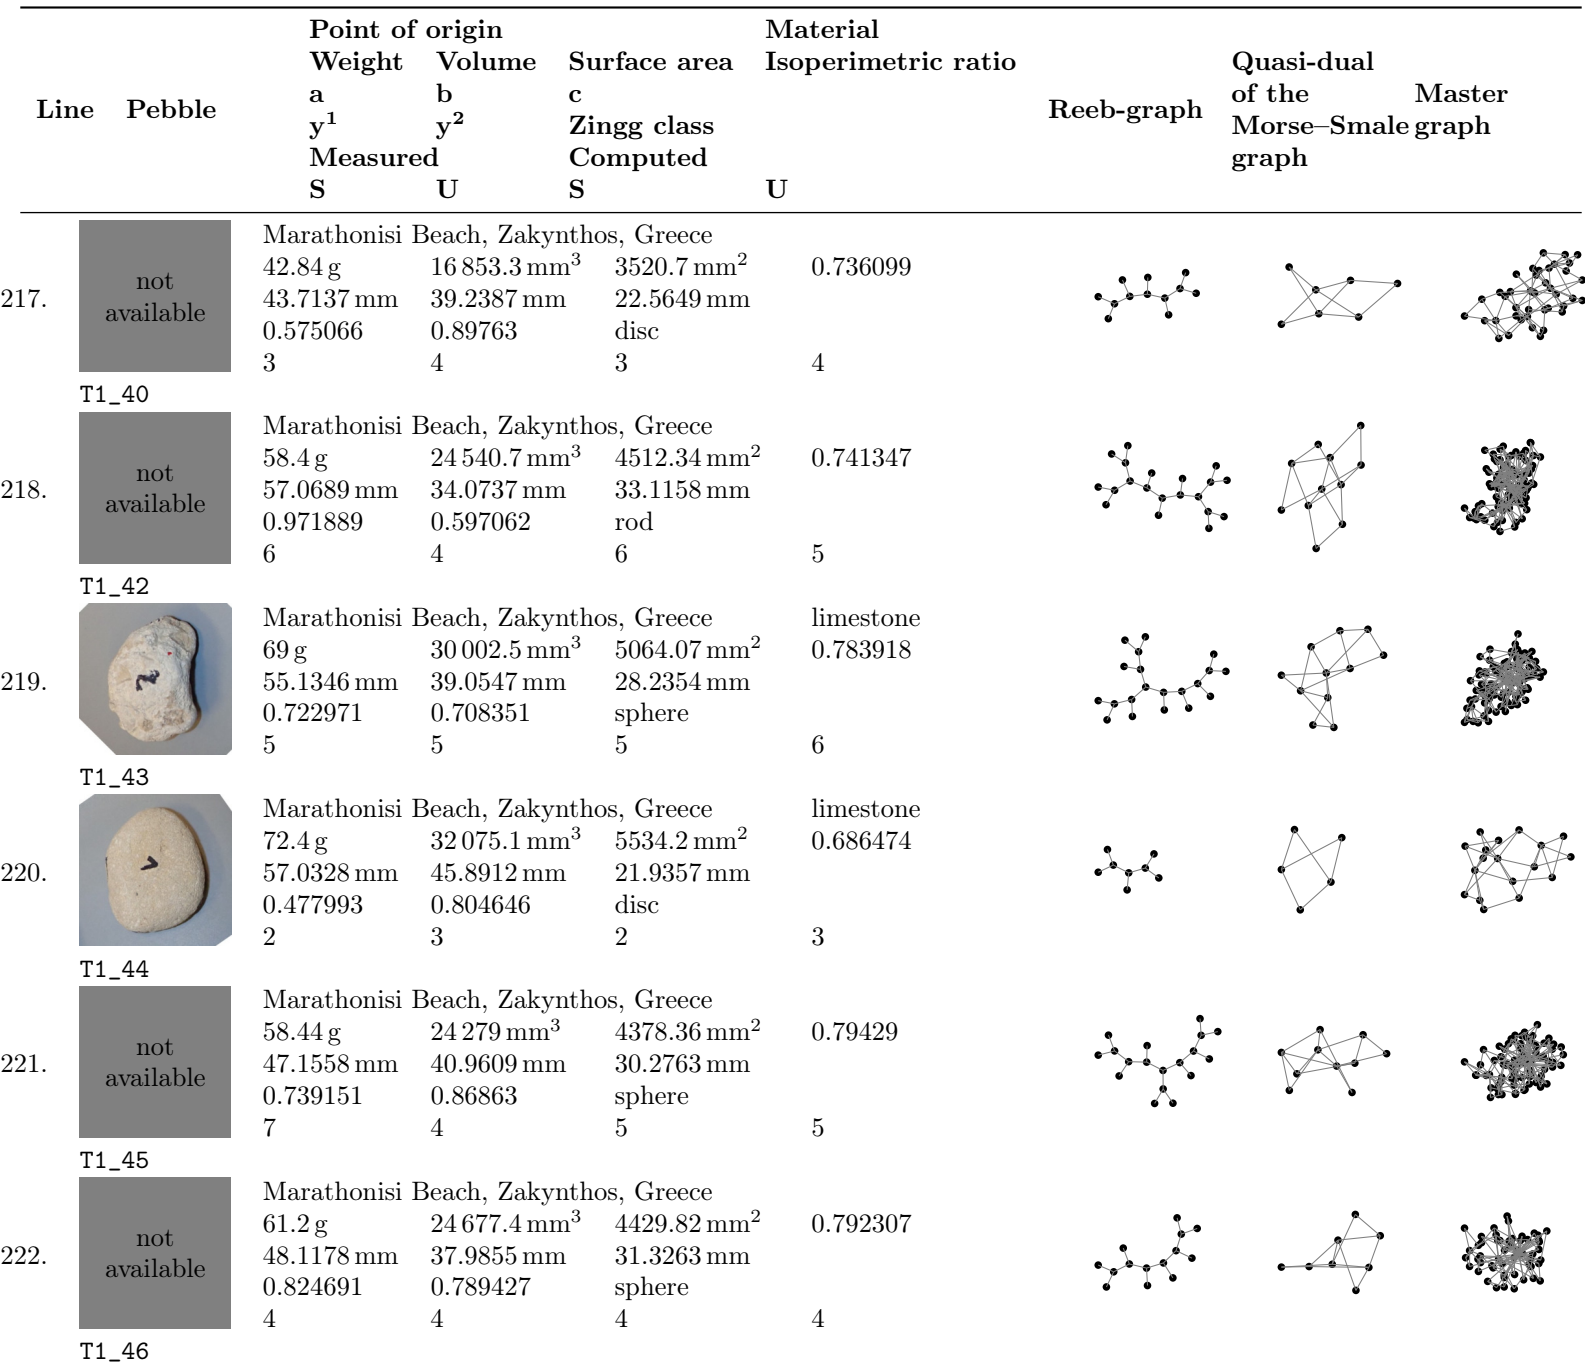   |
|      | T1_42                                                                               |                                                                                |                                                         |                                                      |                                      |                                                                                       |                                                                                       |                                                                                       |
| 219. | 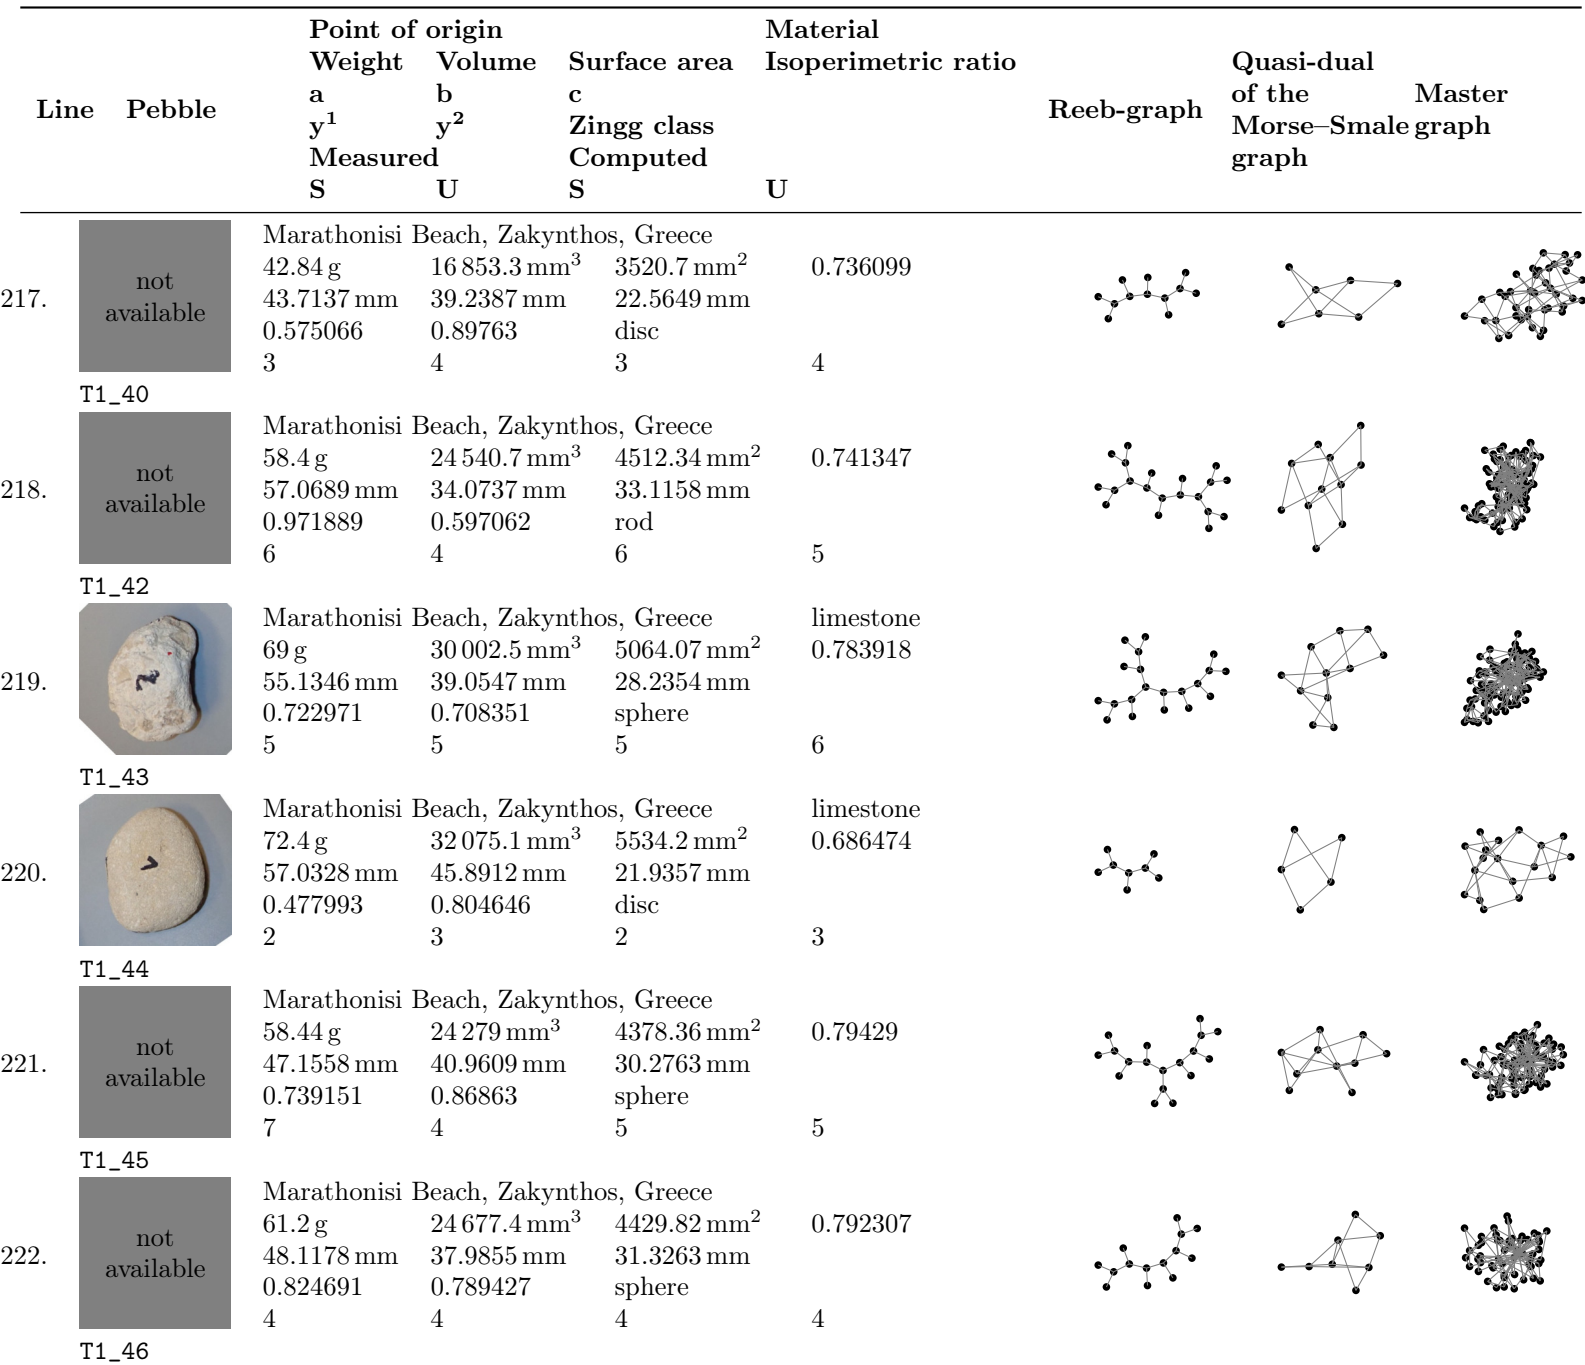   | Marathonisi Beach, Zakynthos, Greece<br>69 g<br>55.1346 mm<br>0.722971<br>5    | 30 002.5 mm <sup>3</sup><br>39.0547 mm<br>0.708351<br>5 | 5064.07 mm <sup>2</sup><br>28.2354 mm<br>sphere<br>5 | limestone<br>0.783918<br><br><br>6   | 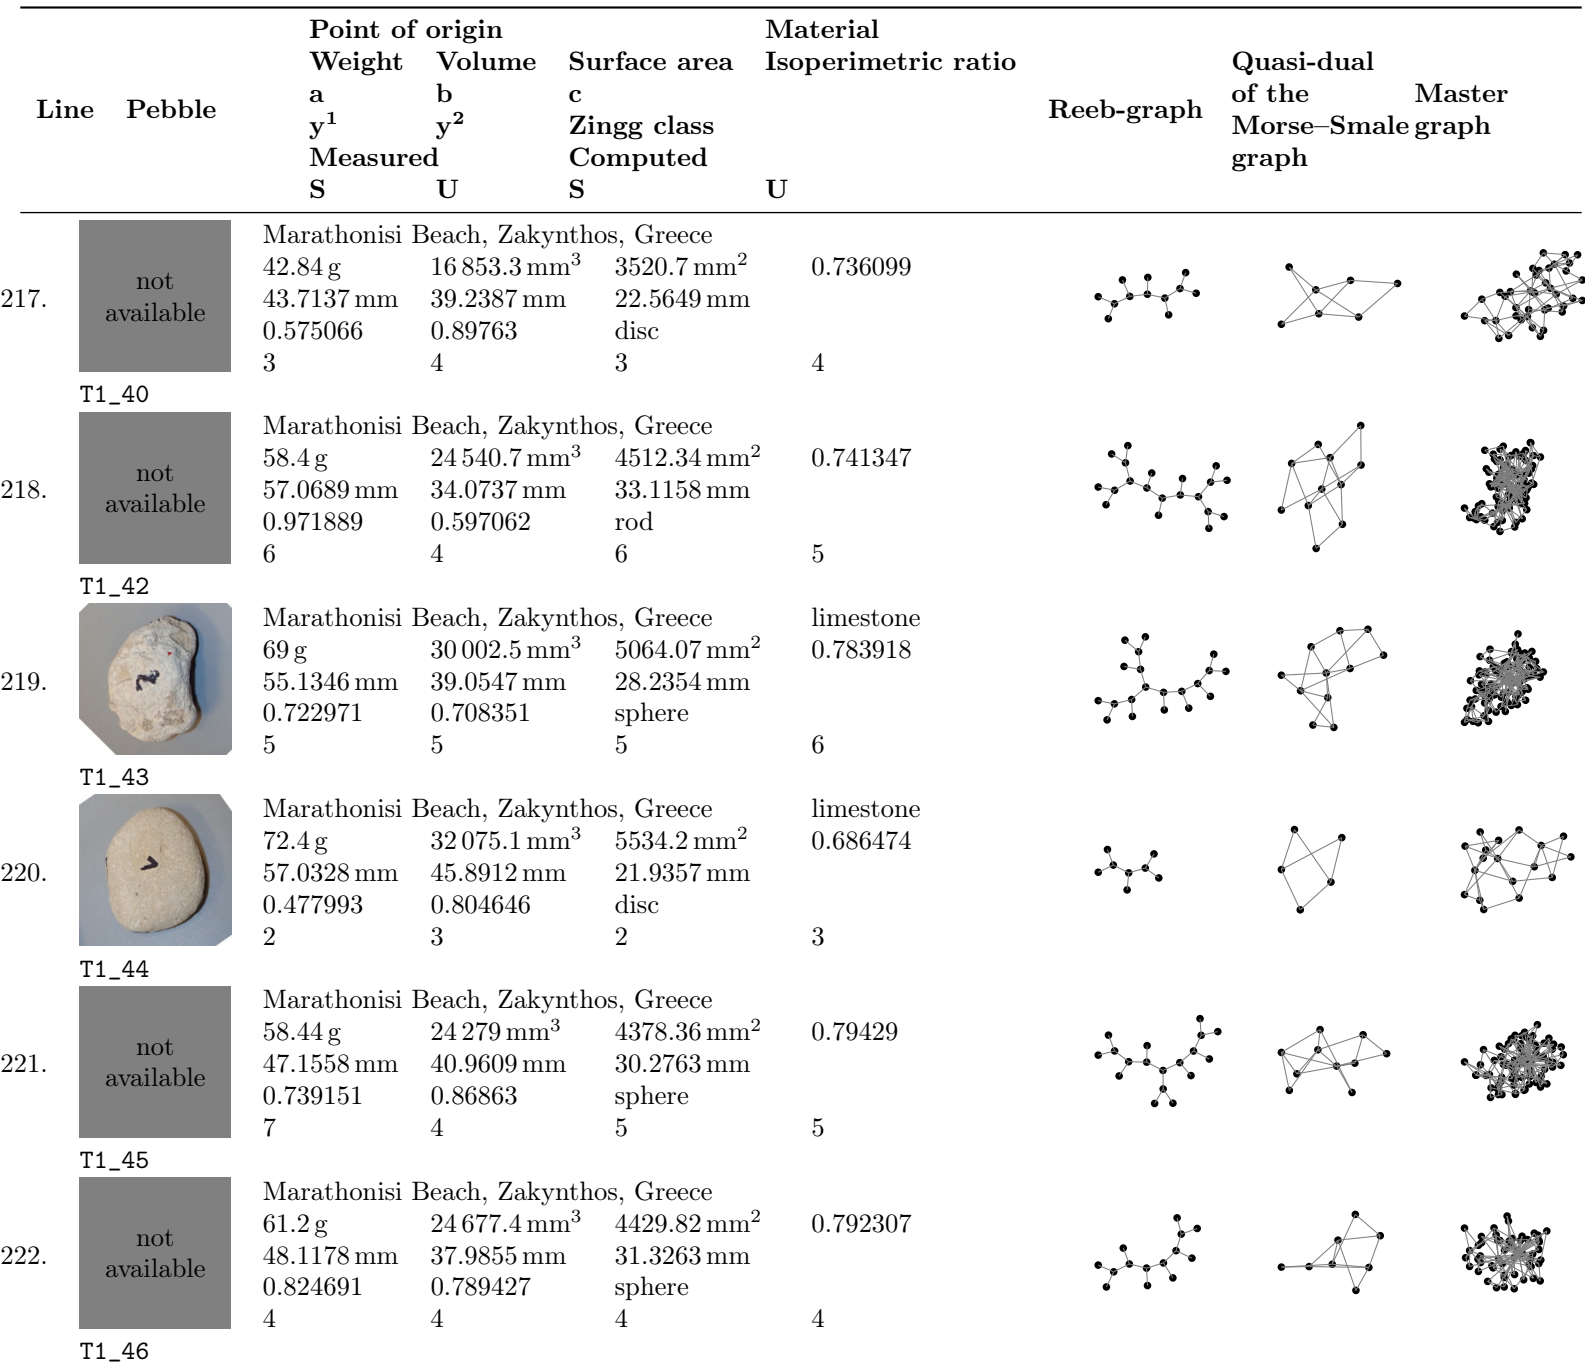   | 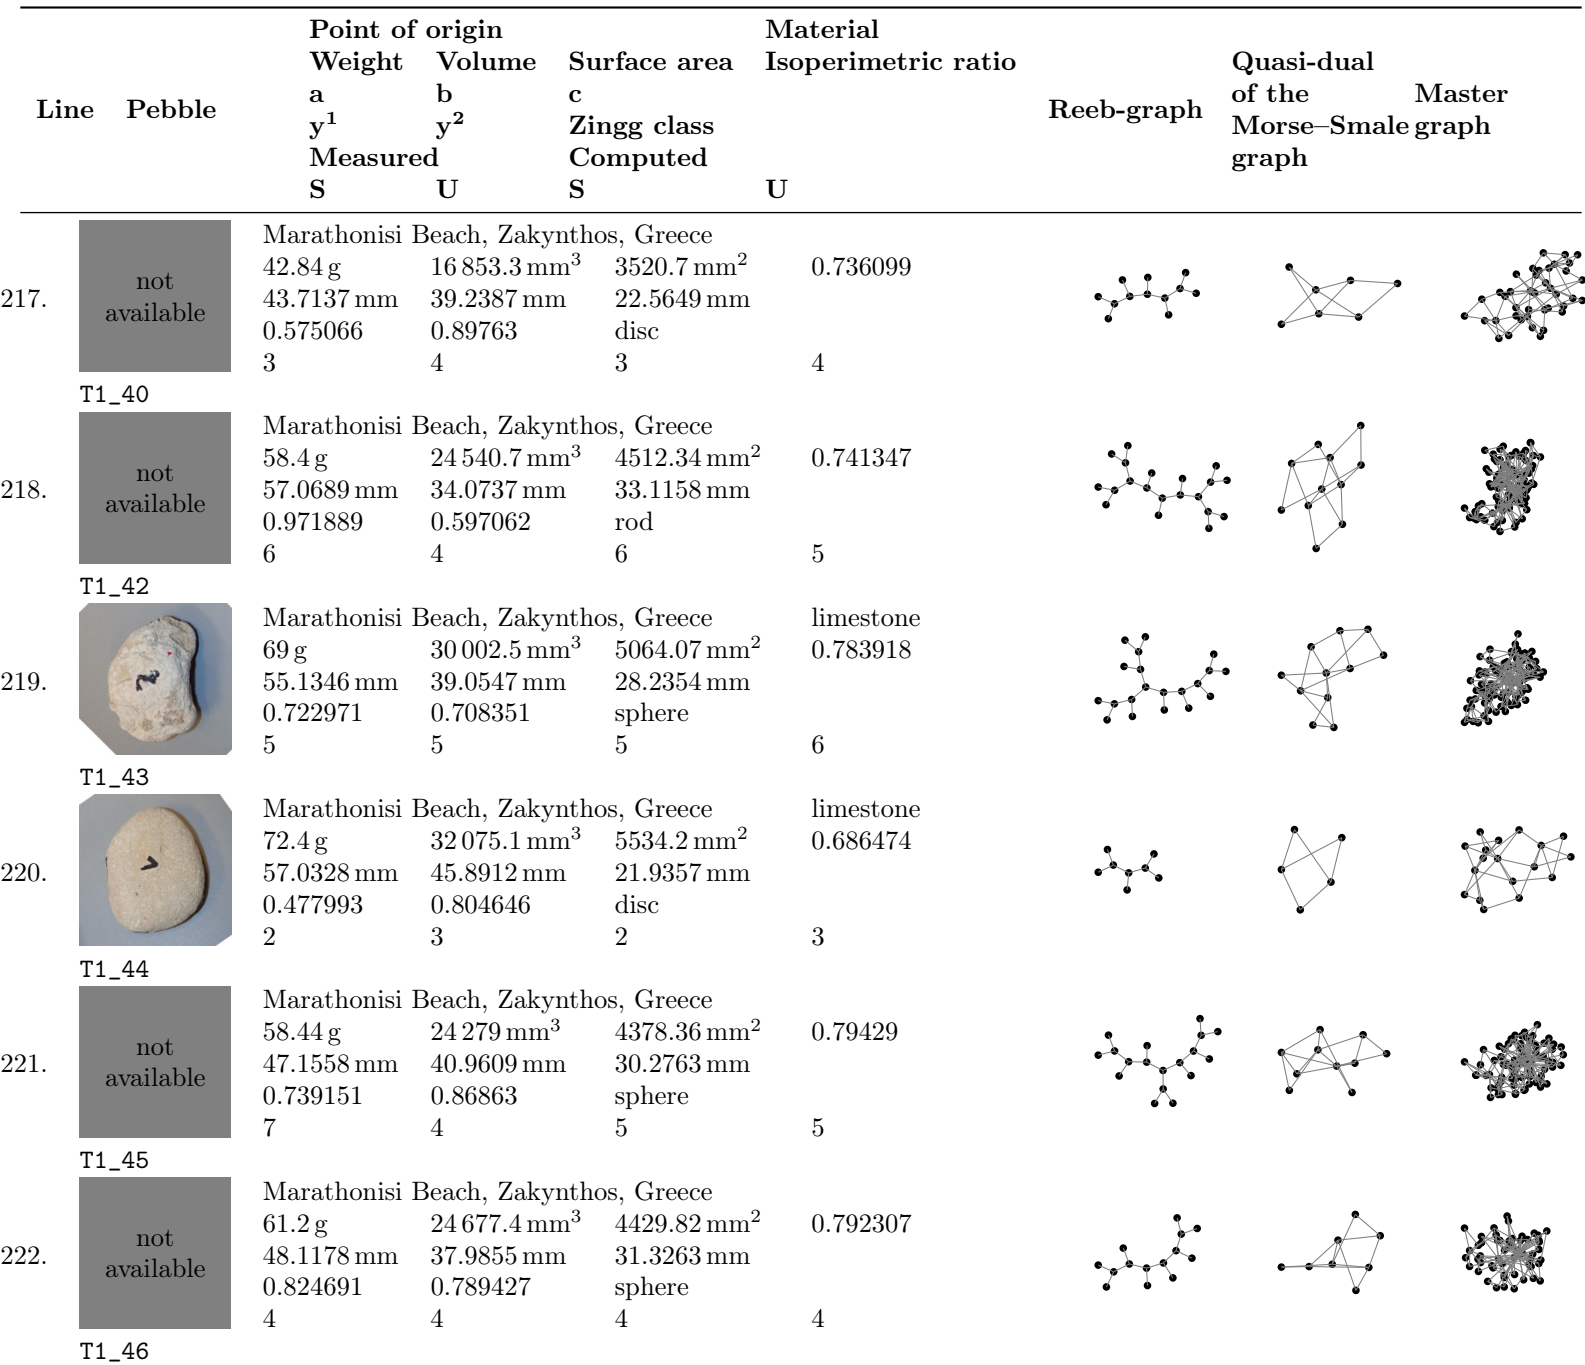   | 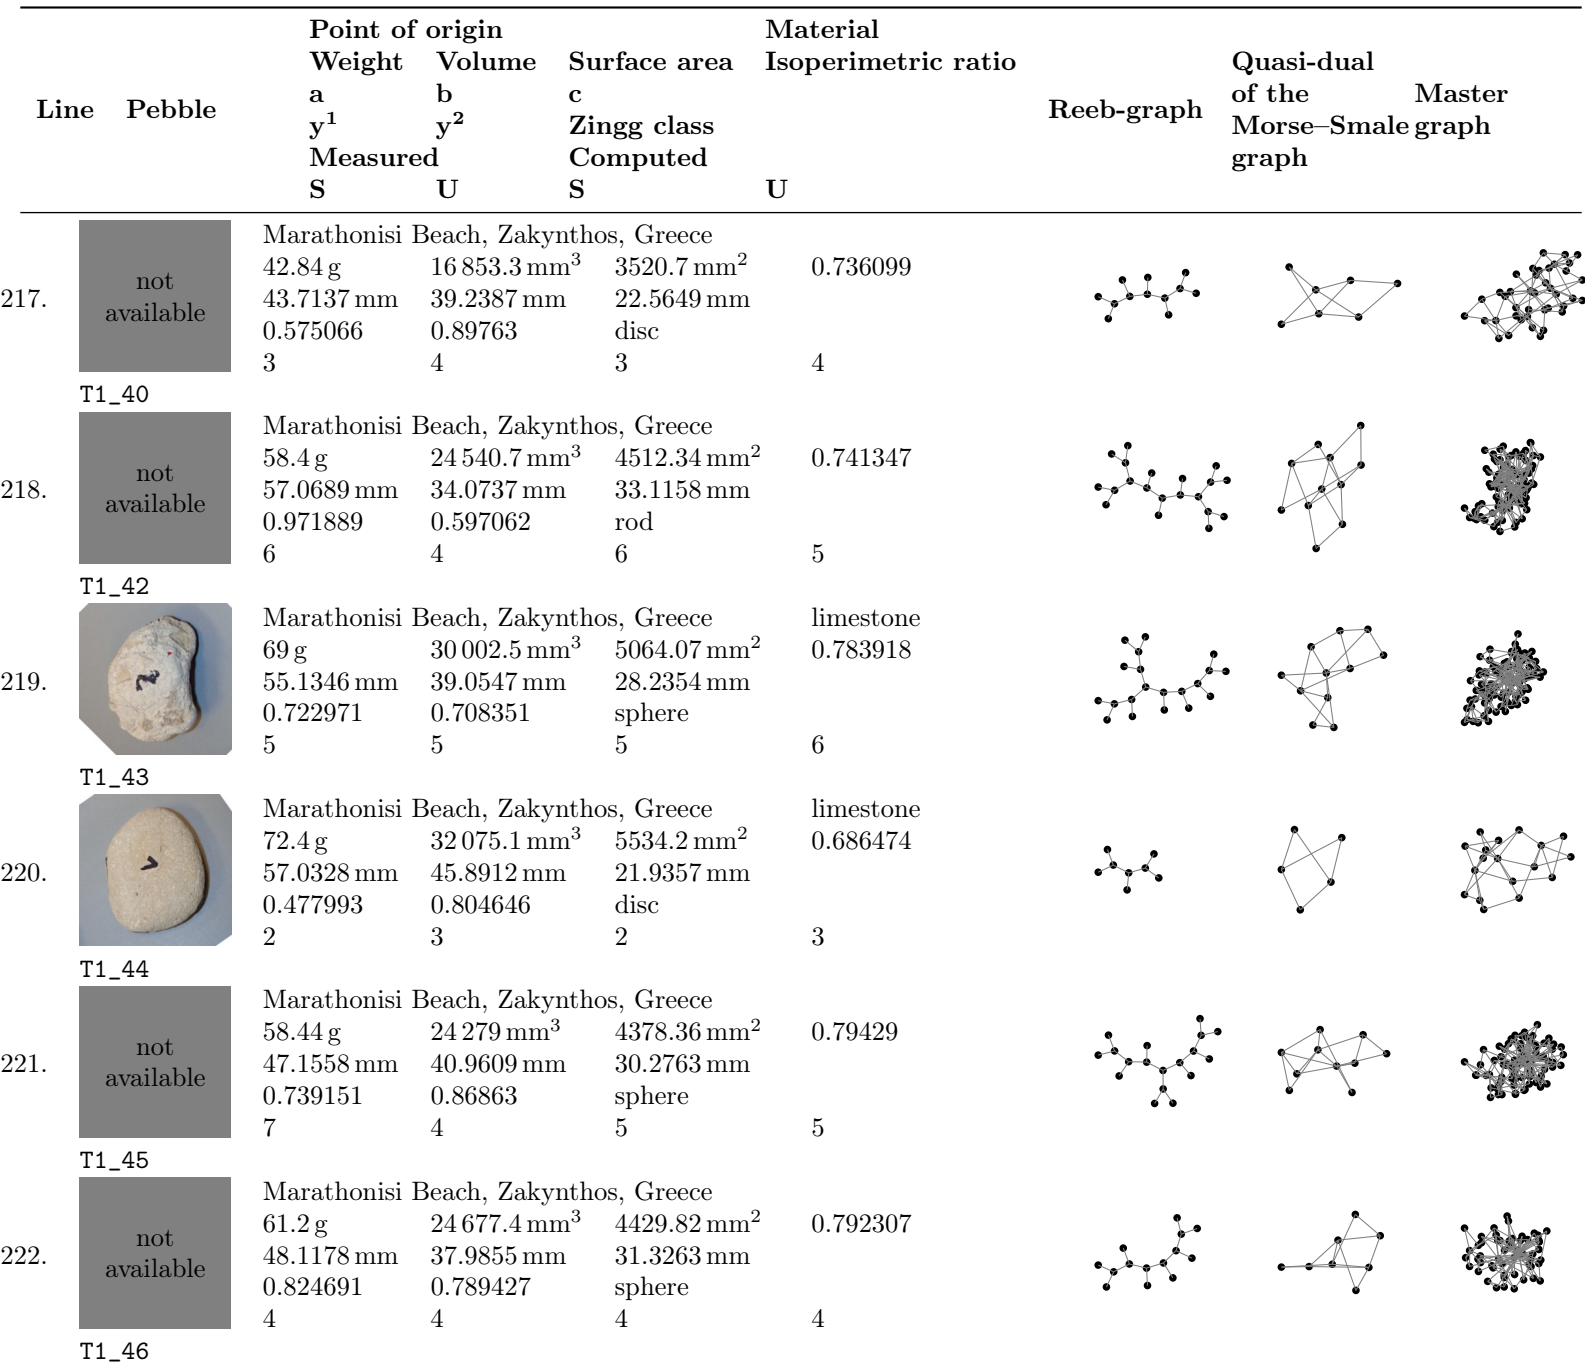   |
|      | T1_43                                                                               |                                                                                |                                                         |                                                      |                                      |                                                                                       |                                                                                       |                                                                                       |
| 220. | 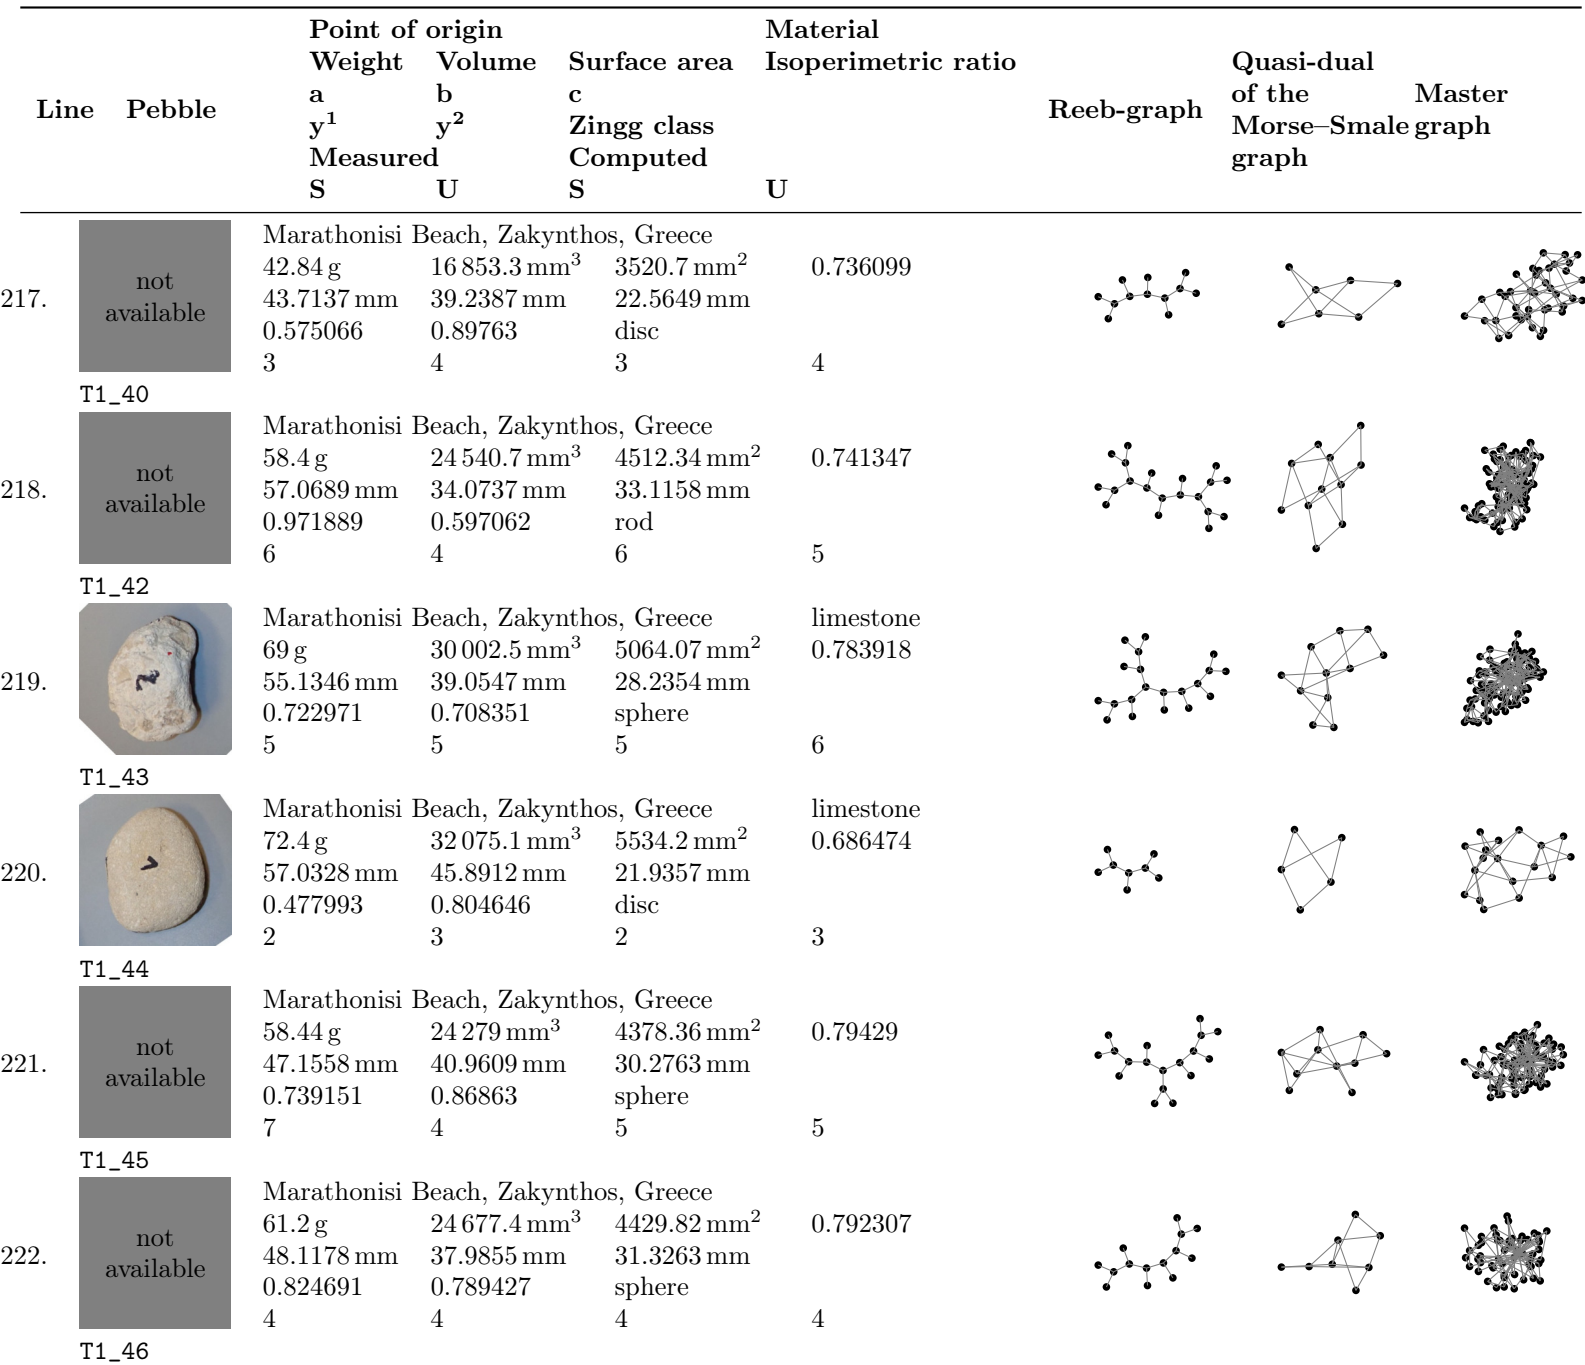  | Marathonisi Beach, Zakynthos, Greece<br>72.4 g<br>57.0328 mm<br>0.477993<br>2  | 32 075.1 mm <sup>3</sup><br>45.8912 mm<br>0.804646<br>3 | 5534.2 mm <sup>2</sup><br>21.9357 mm<br>disc<br>2    | limestone<br>0.686474<br><br><br>3   | 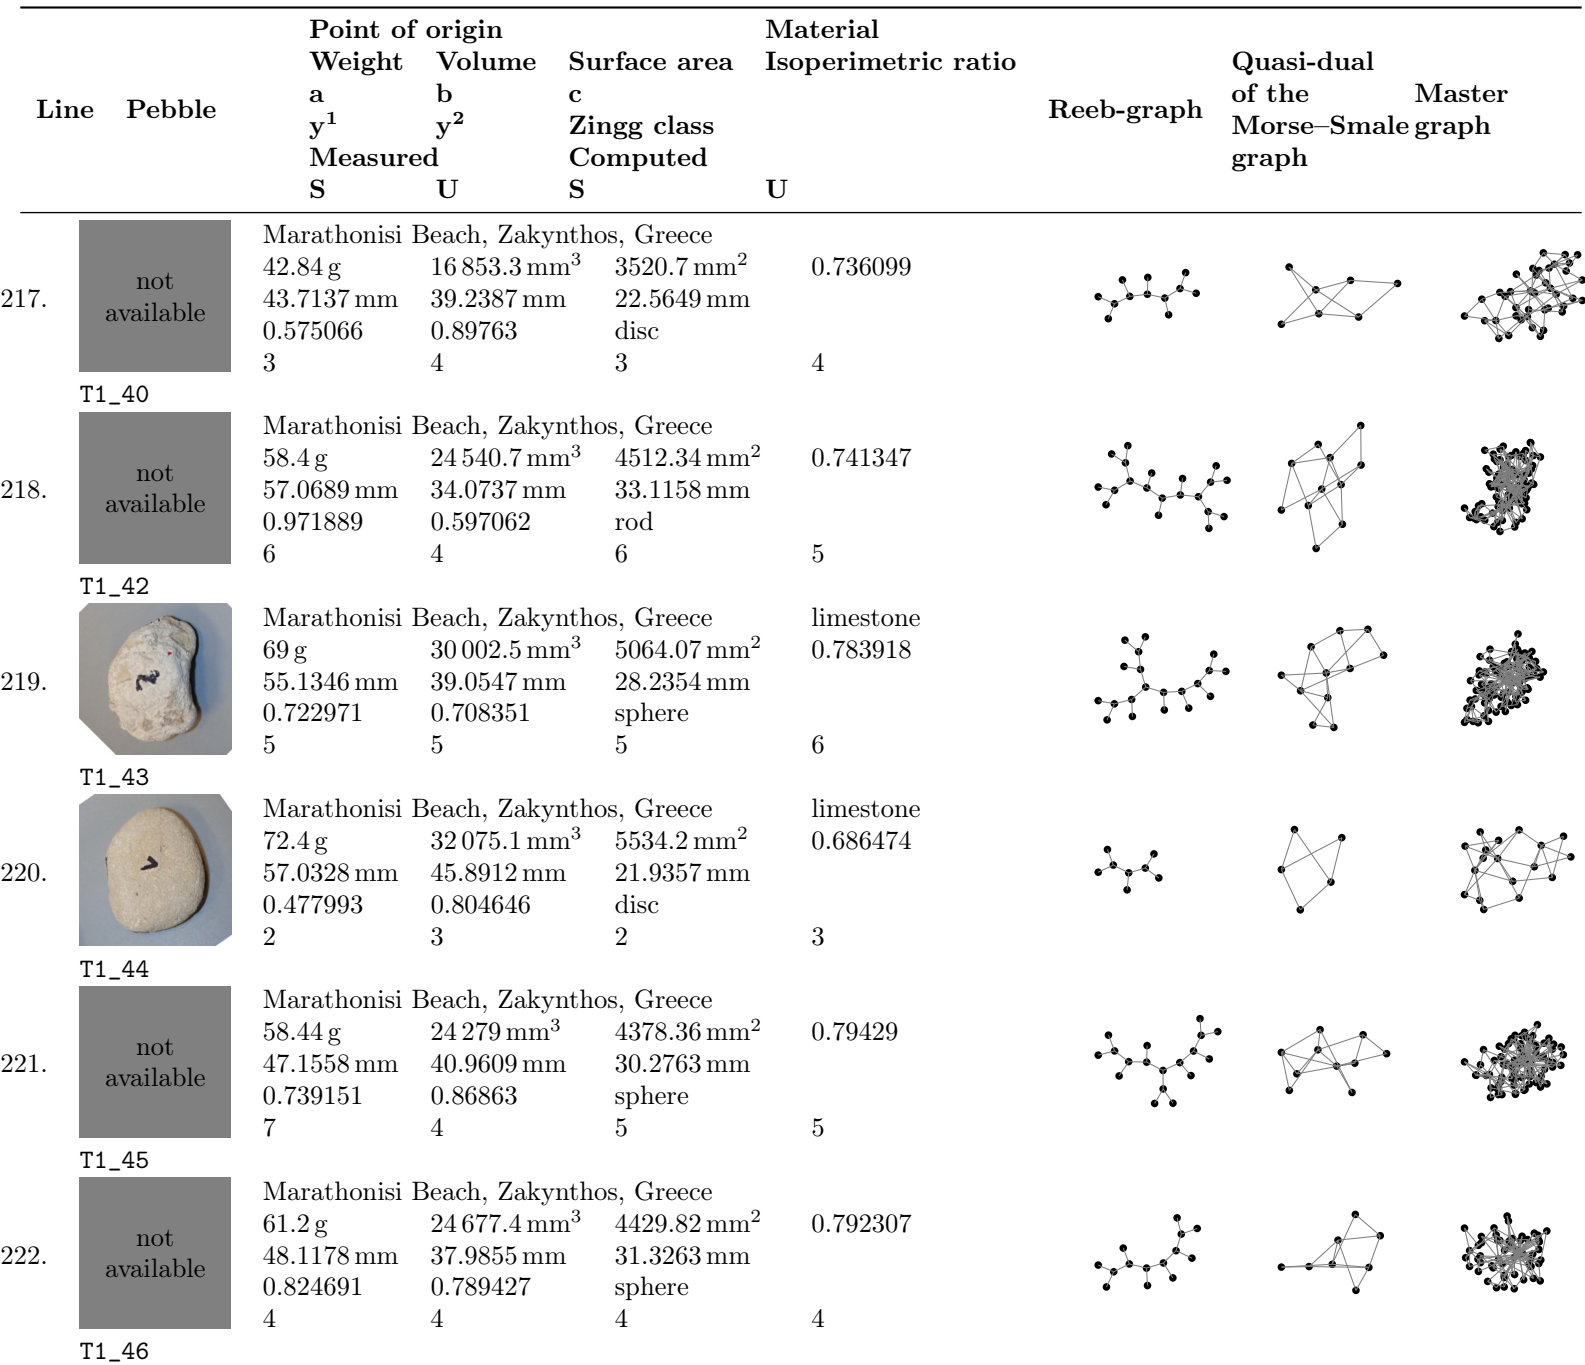  | 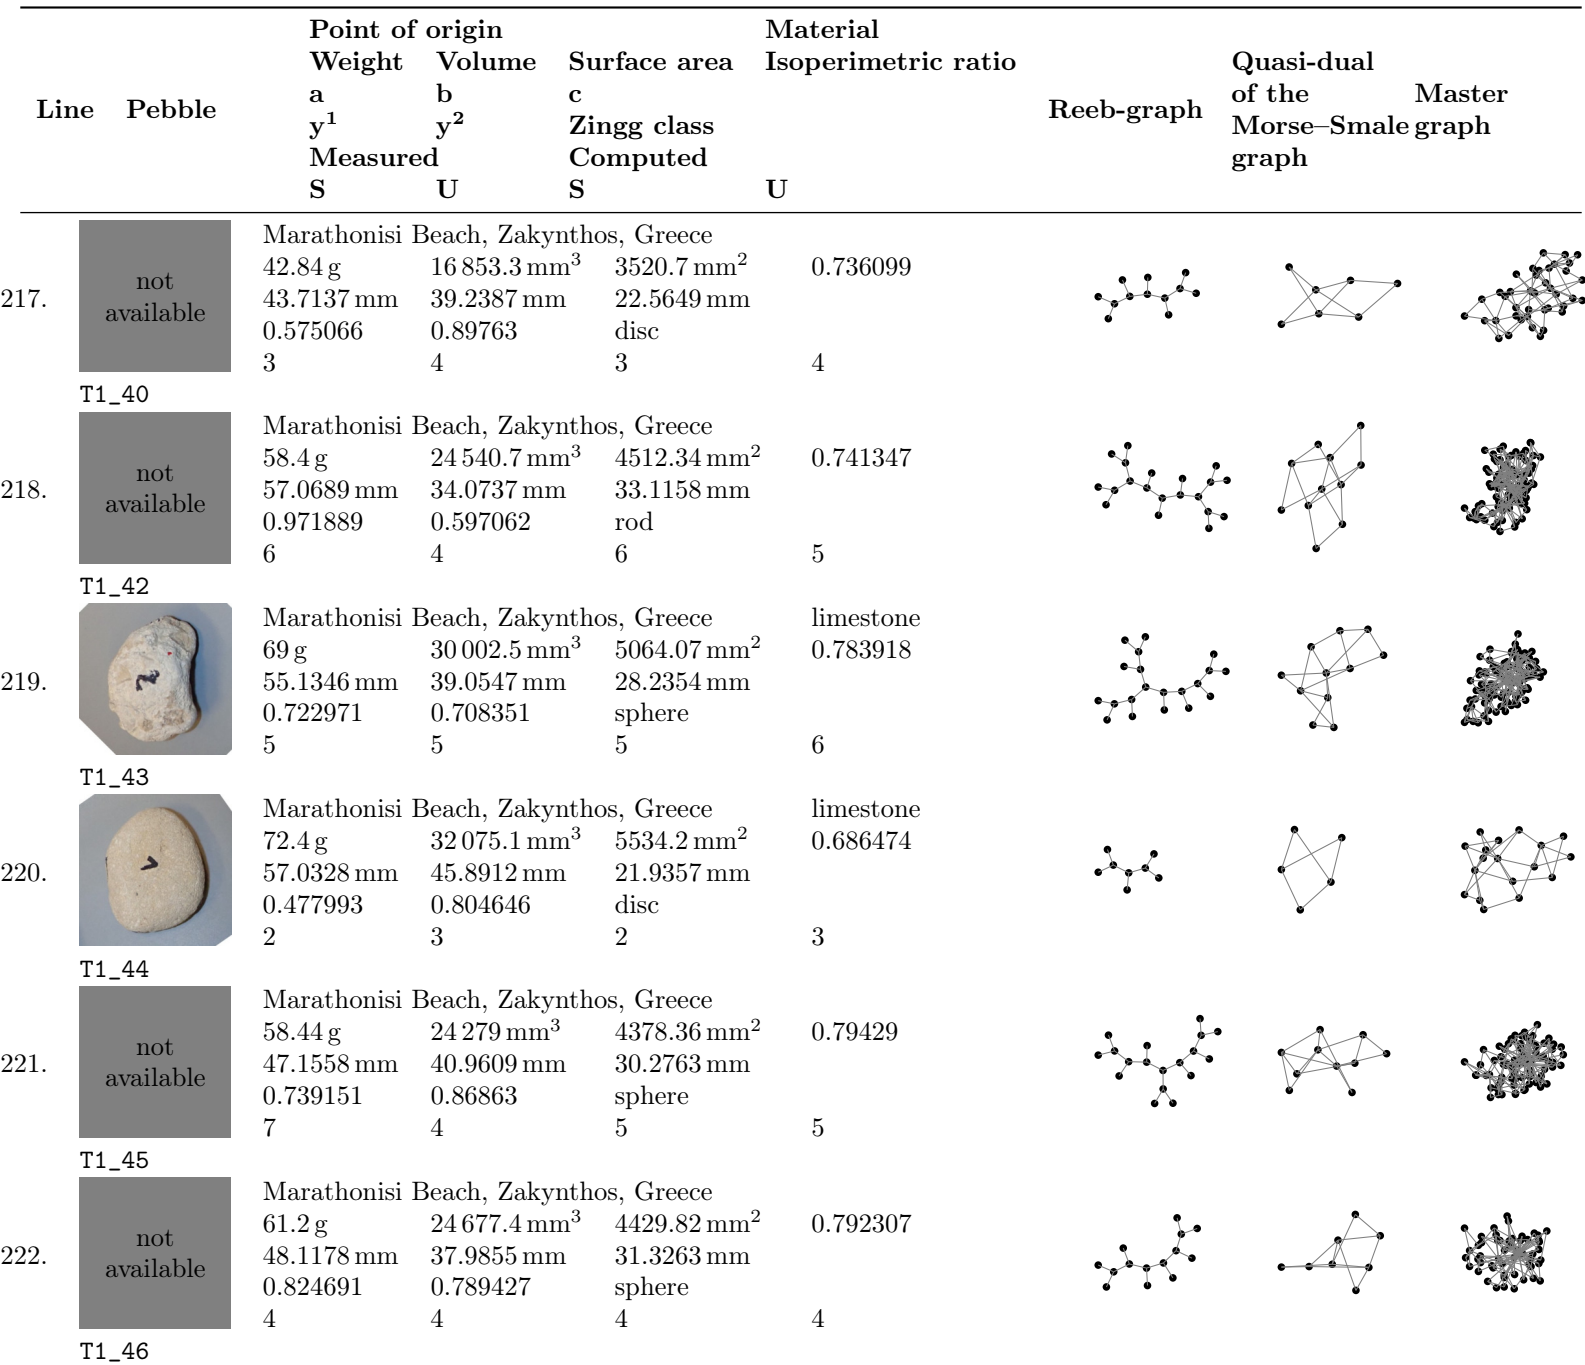  | 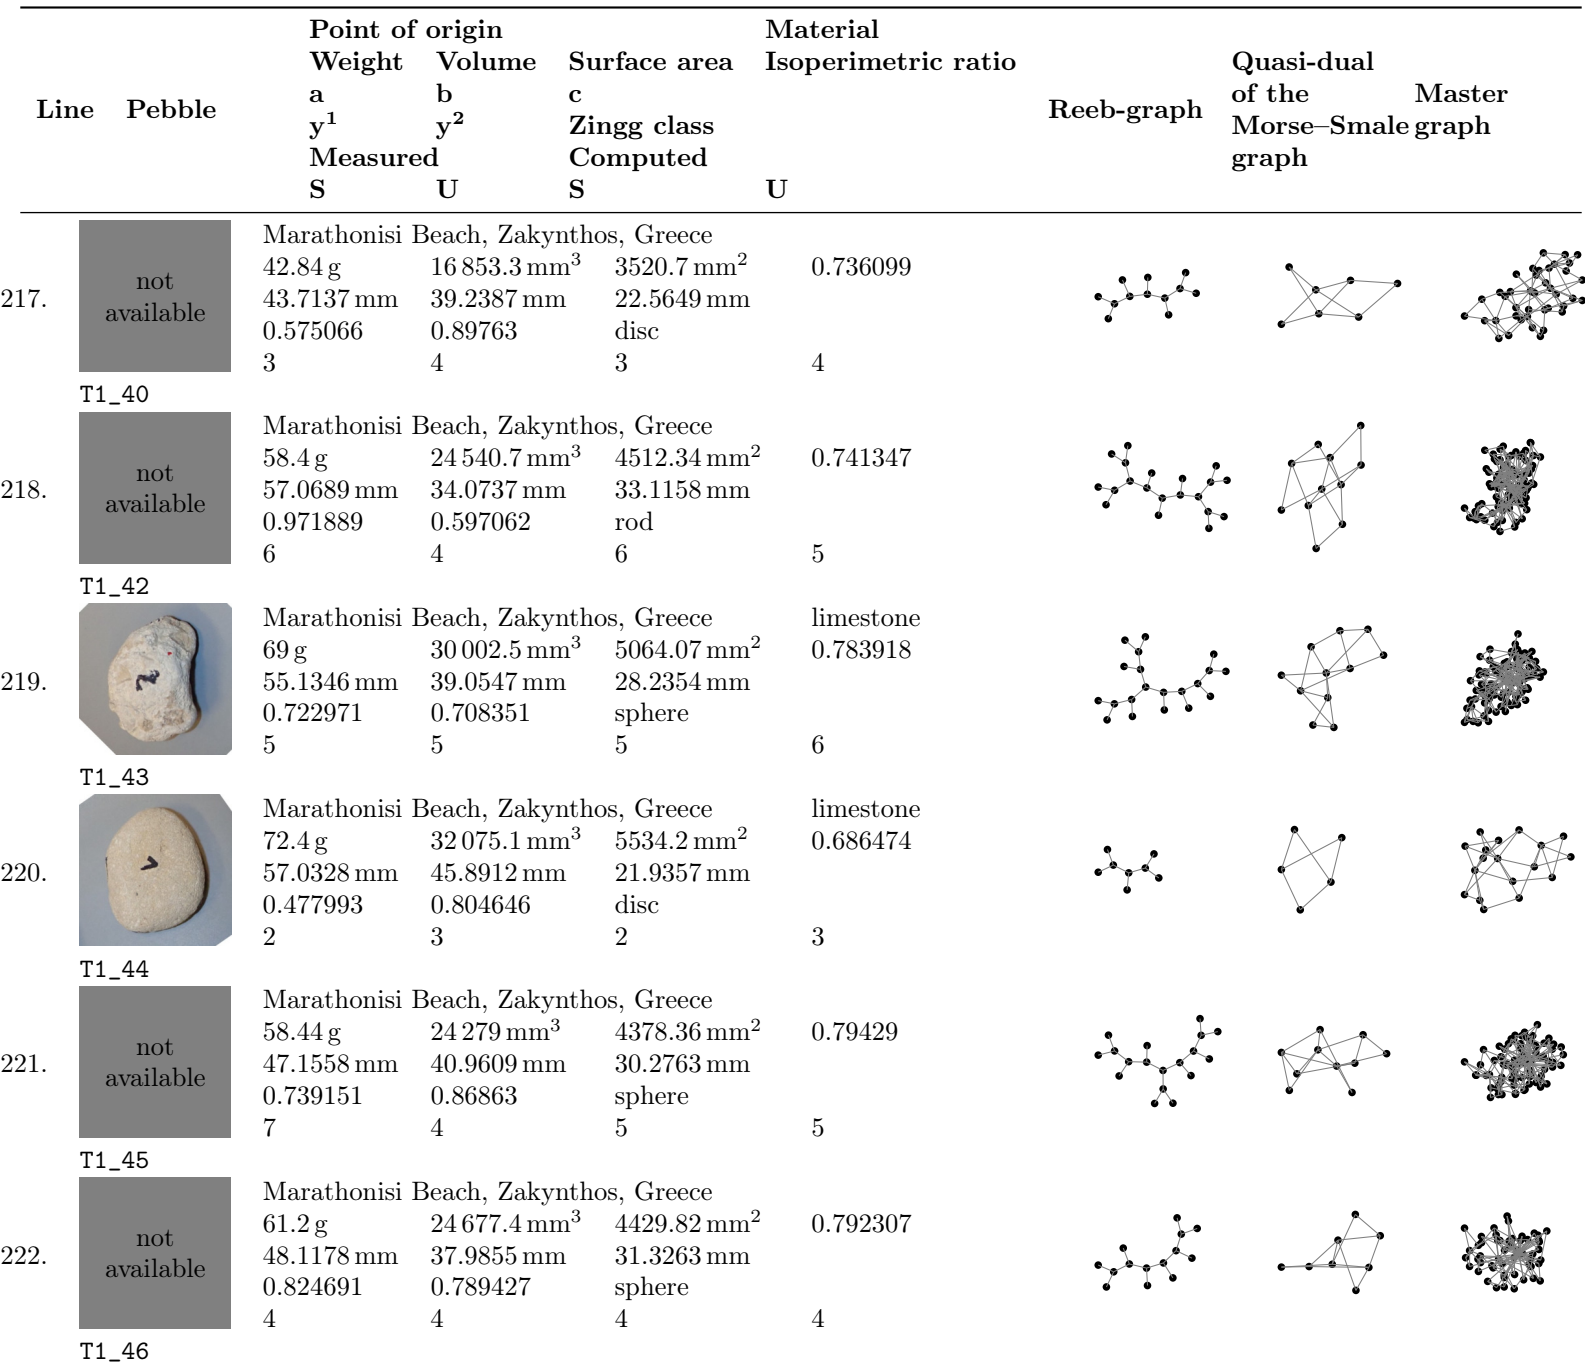  |
|      | T1_44                                                                               |                                                                                |                                                         |                                                      |                                      |                                                                                       |                                                                                       |                                                                                       |
| 221. | 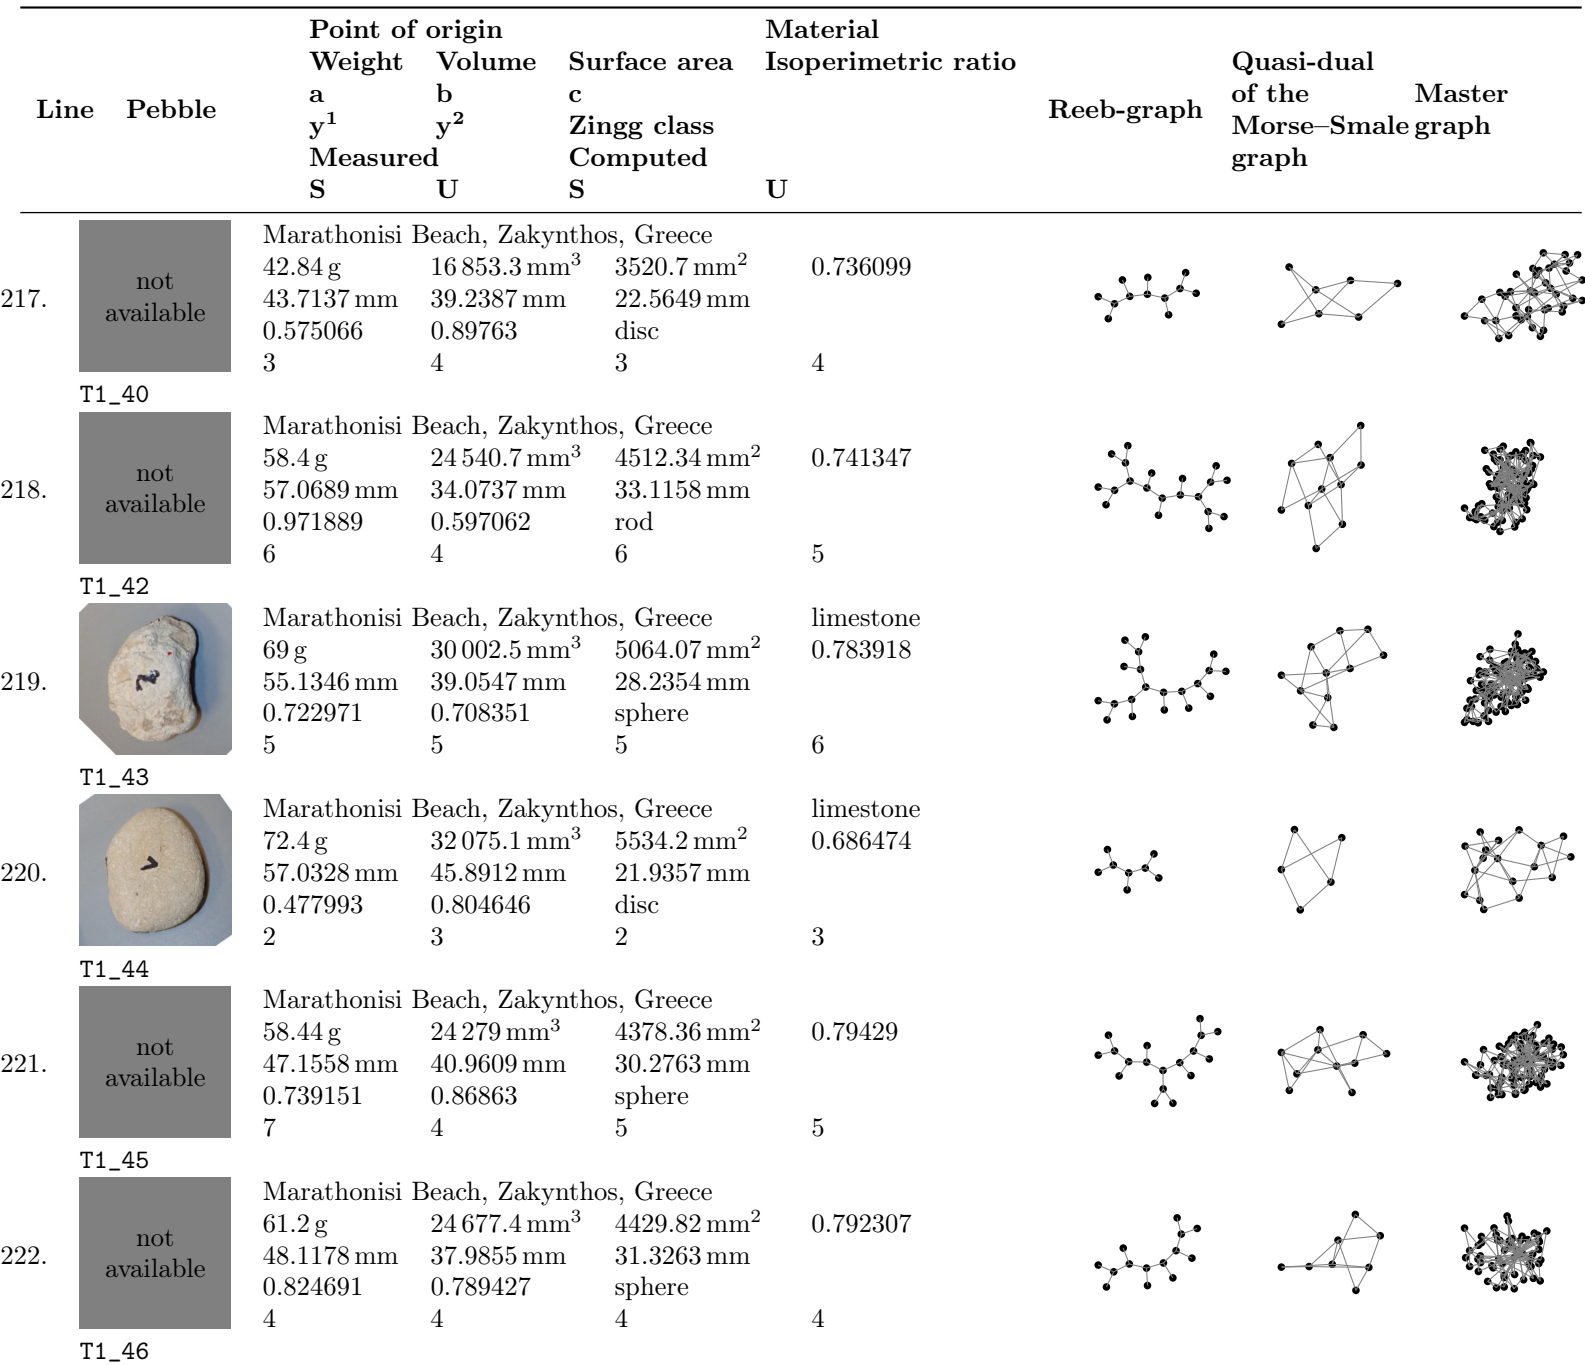 | Marathonisi Beach, Zakynthos, Greece<br>58.44 g<br>47.1558 mm<br>0.739151<br>7 | 24 279 mm <sup>3</sup><br>40.9609 mm<br>0.86863<br>4    | 4378.36 mm <sup>2</sup><br>30.2763 mm<br>sphere<br>5 | 0.79429<br><br><br>5                 | 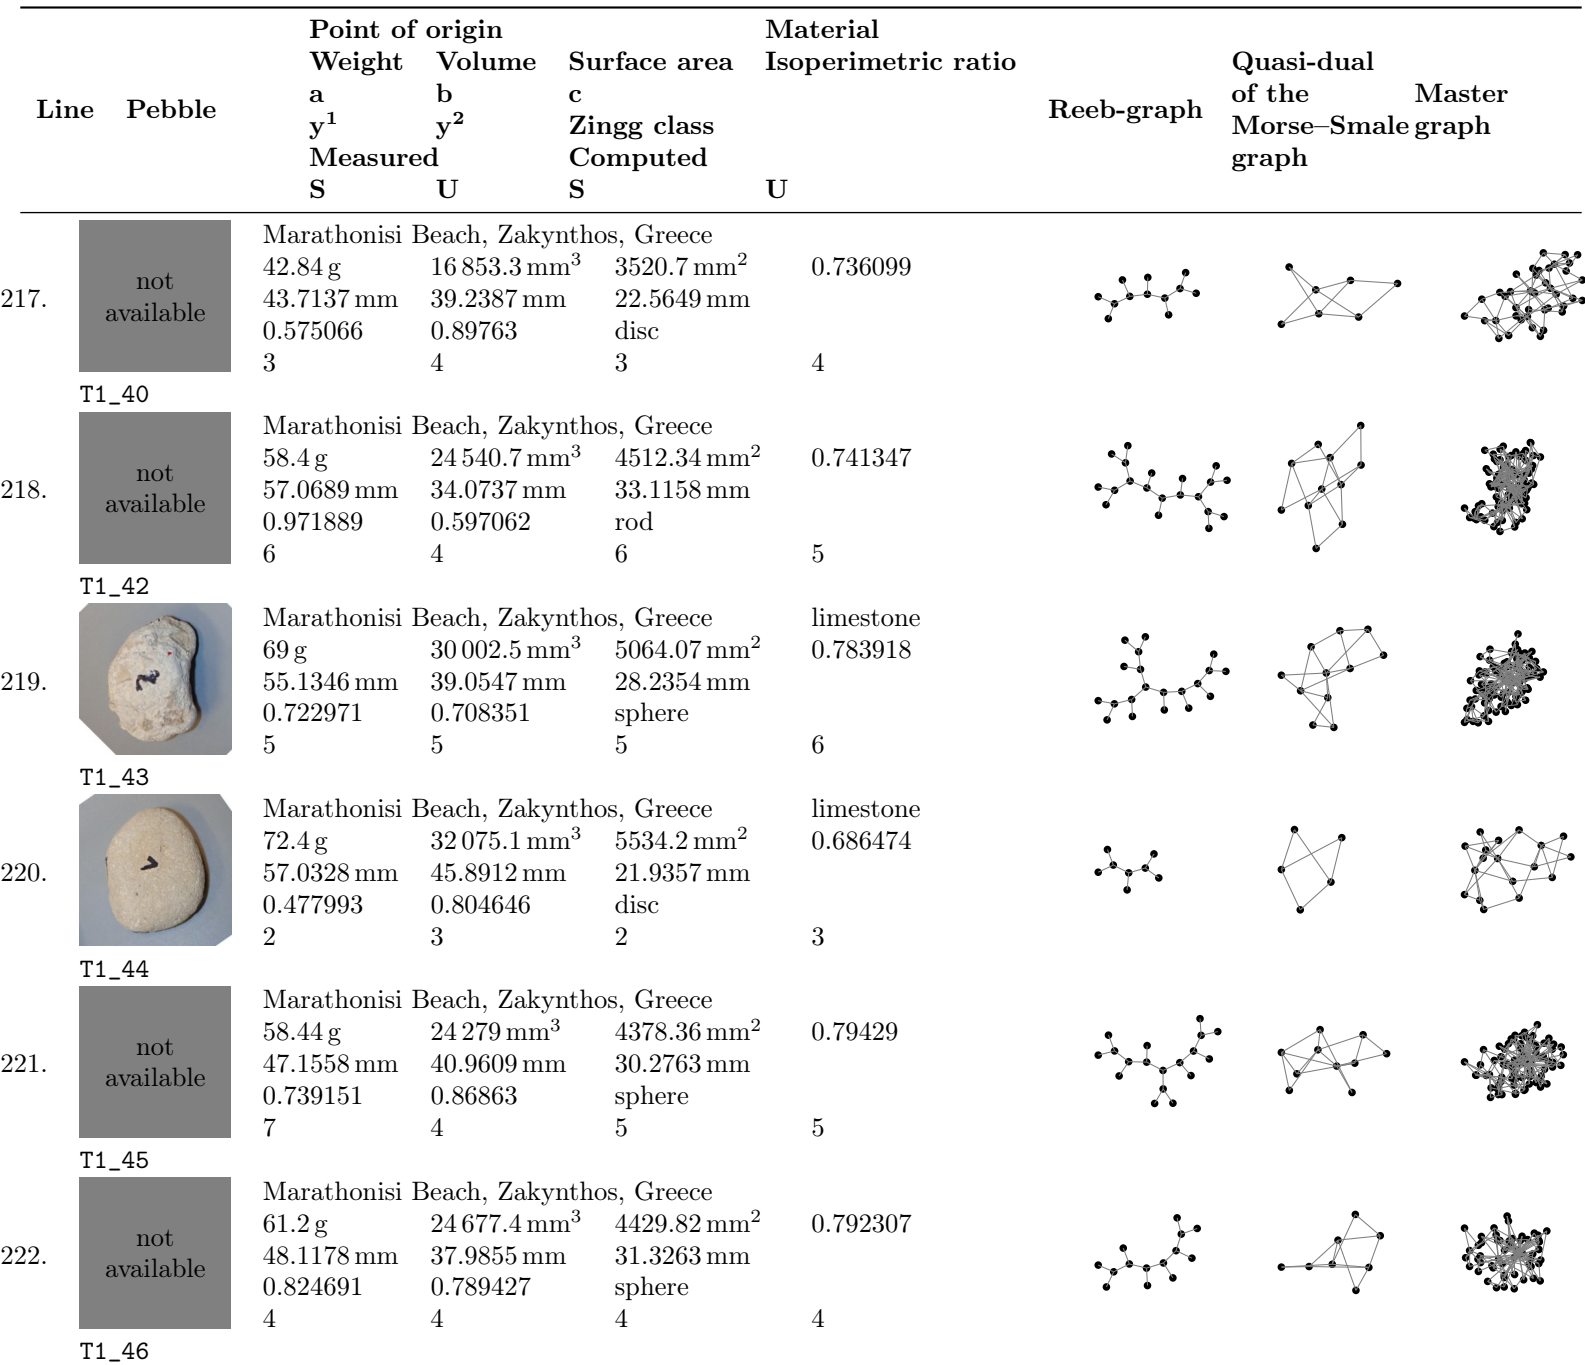 | 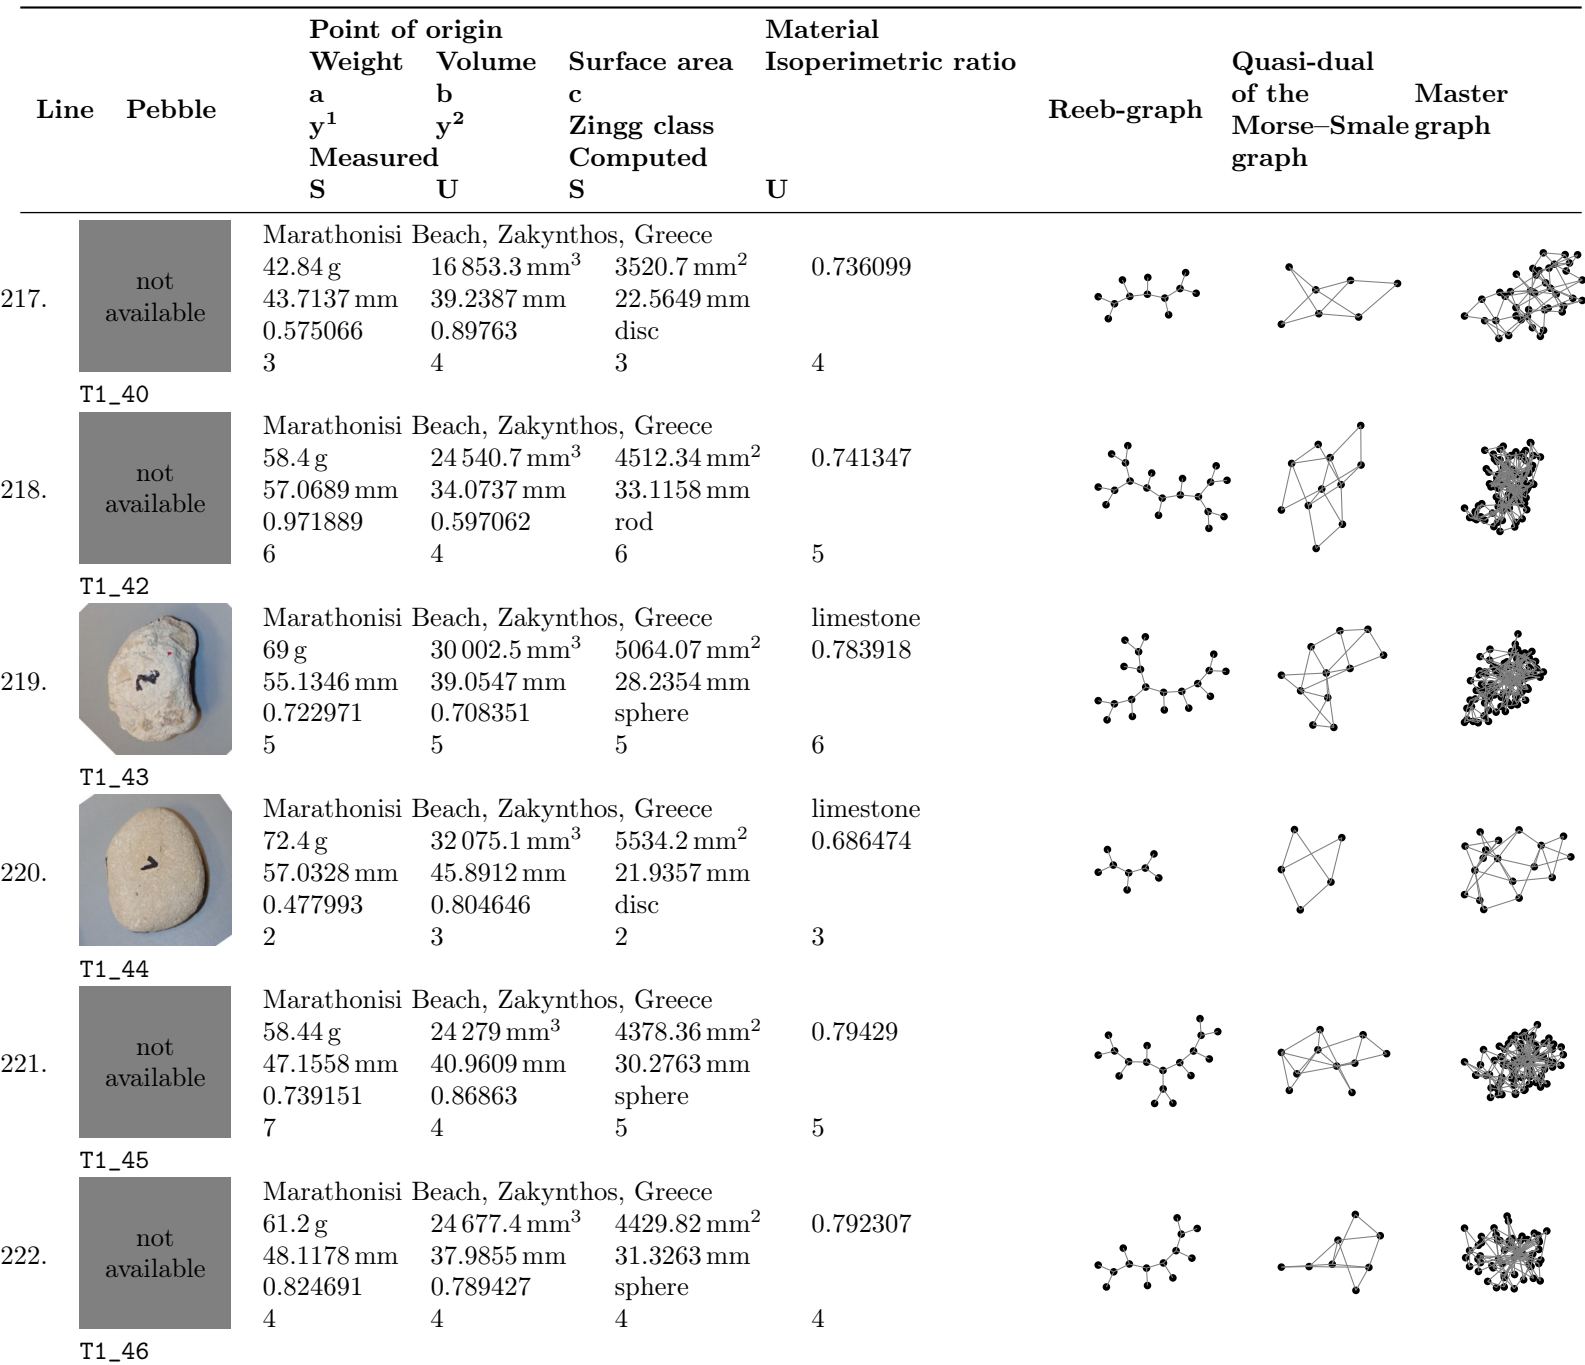 | 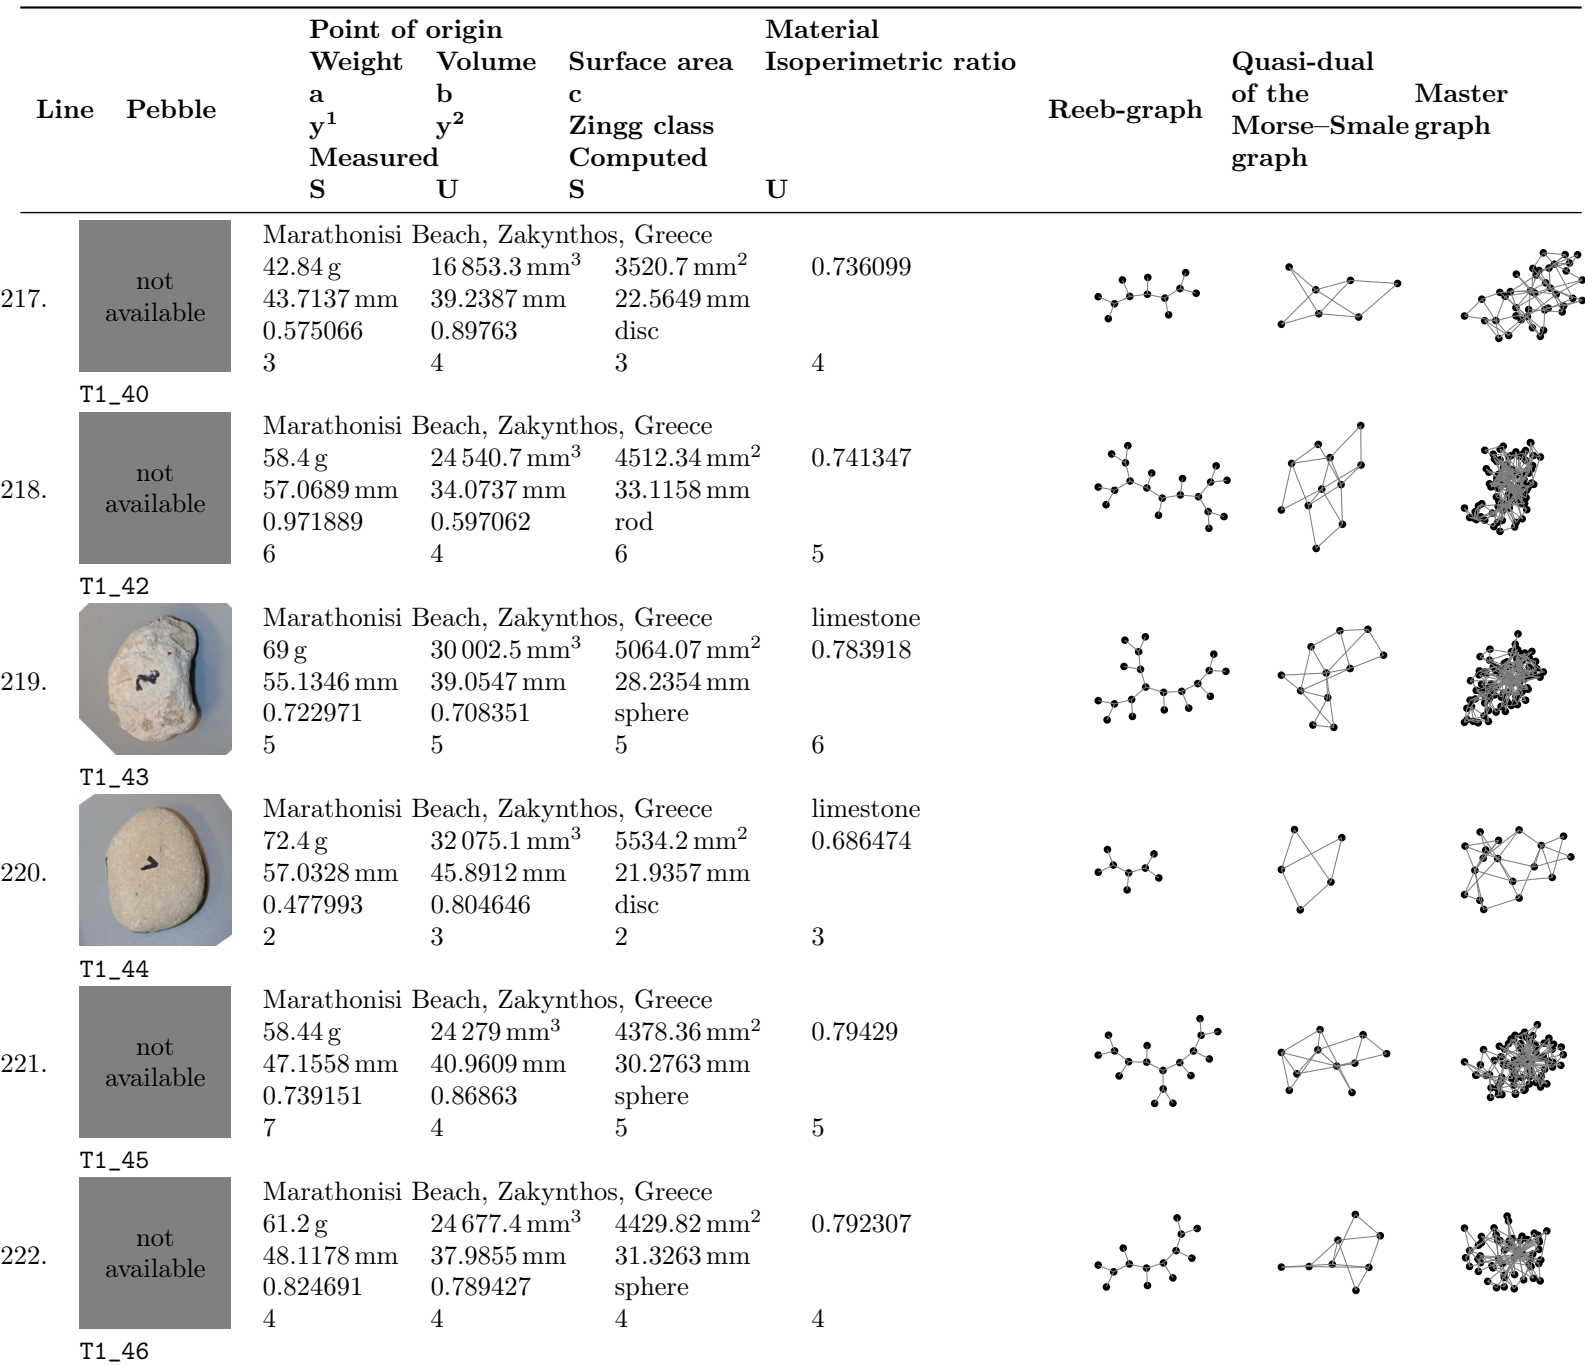 |
|      | T1_45                                                                               |                                                                                |                                                         |                                                      |                                      |                                                                                       |                                                                                       |                                                                                       |
| 222. | 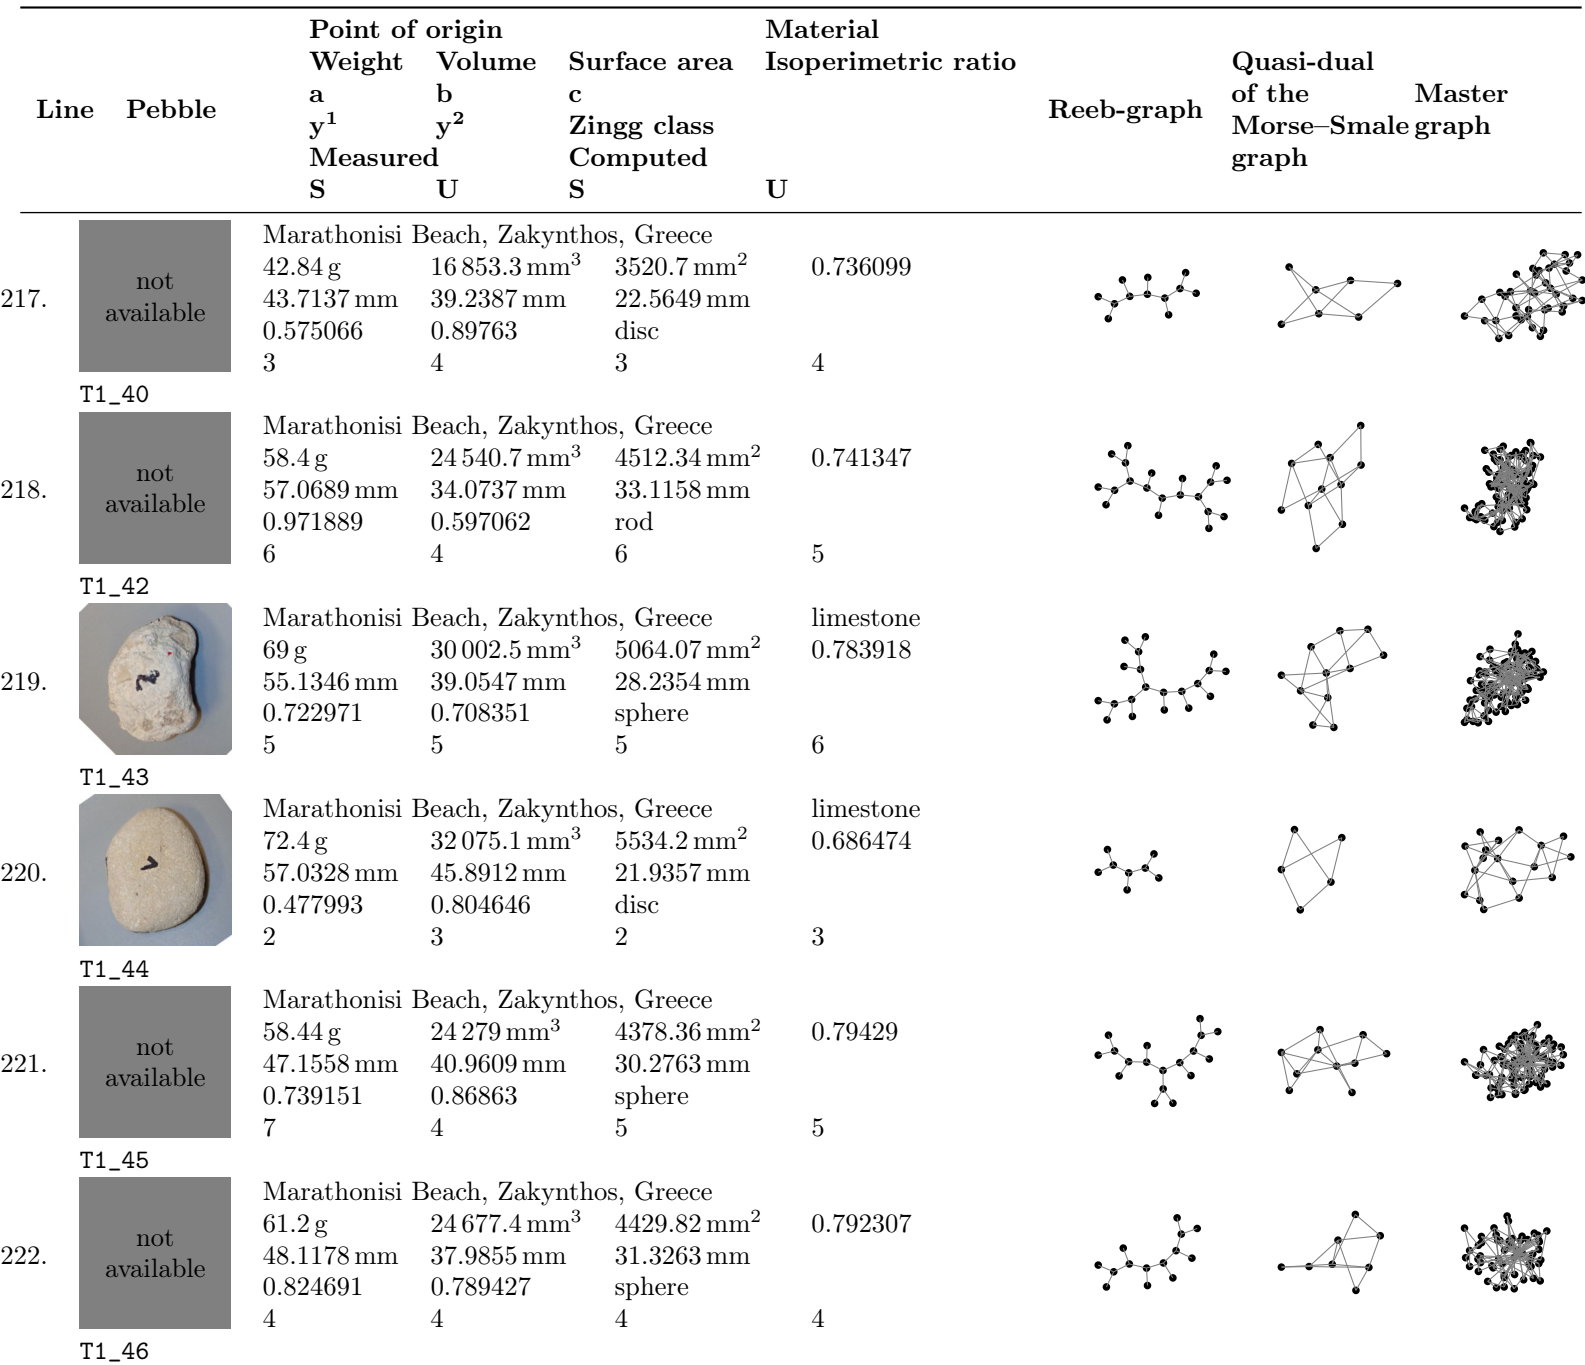 | Marathonisi Beach, Zakynthos, Greece<br>61.2 g<br>48.1178 mm<br>0.824691<br>4  | 24 677.4 mm <sup>3</sup><br>37.9855 mm<br>0.789427<br>4 | 4429.82 mm <sup>2</sup><br>31.3263 mm<br>sphere<br>4 | 0.792307<br><br><br>4                | 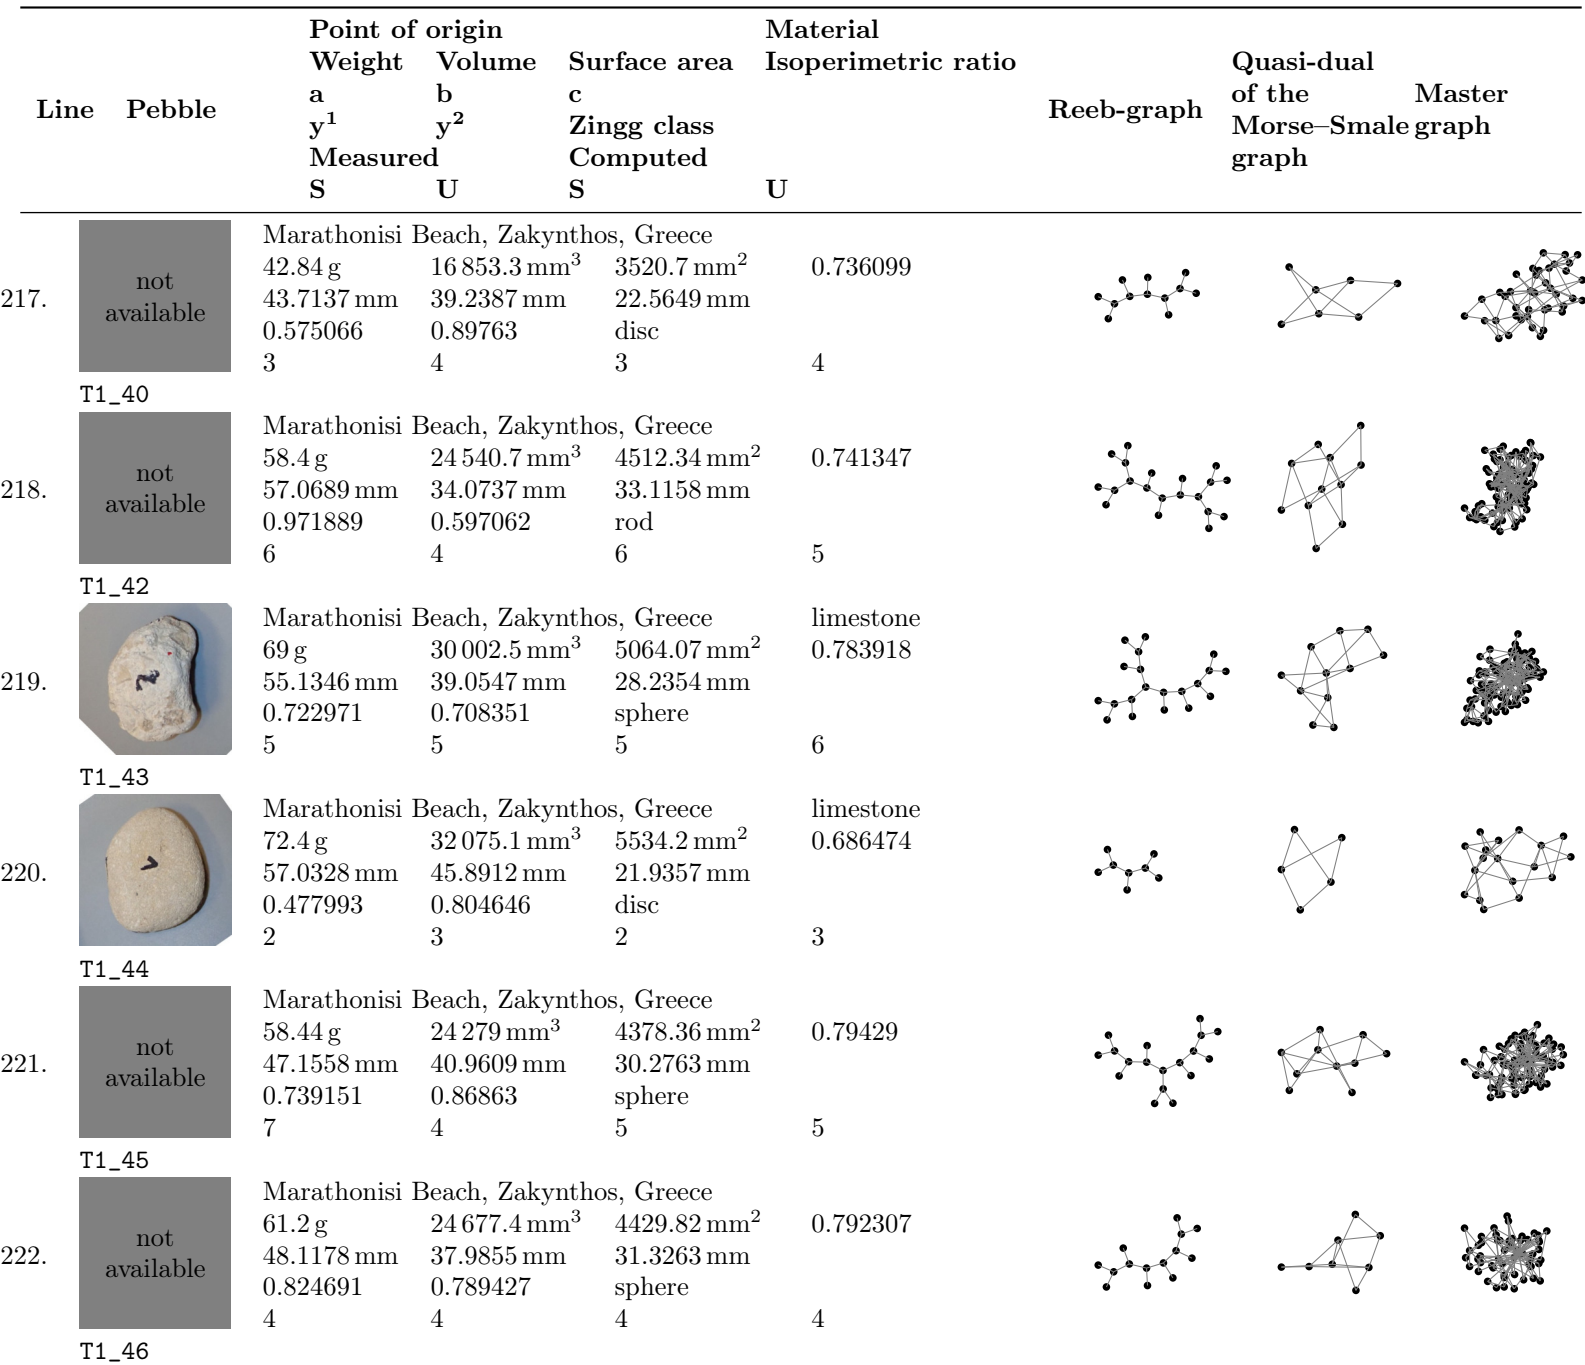 | 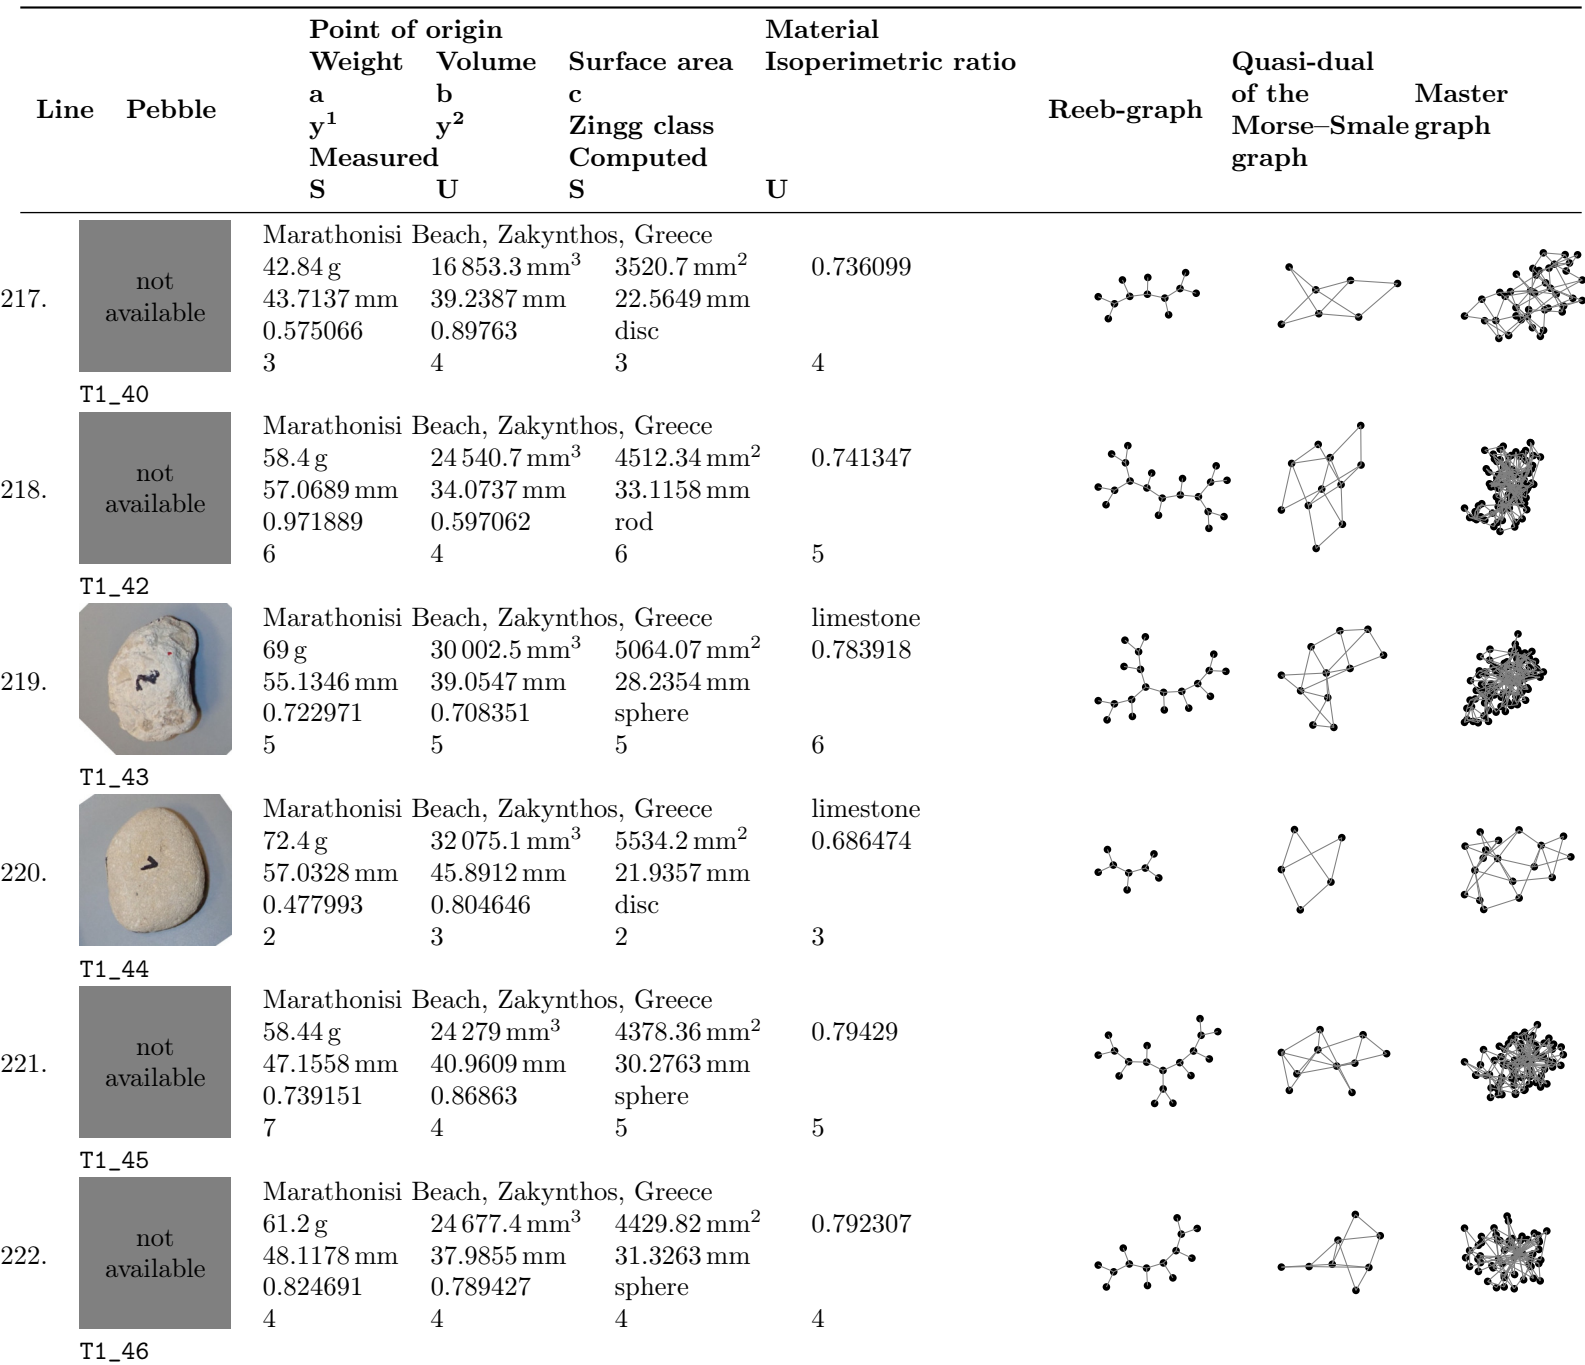 | 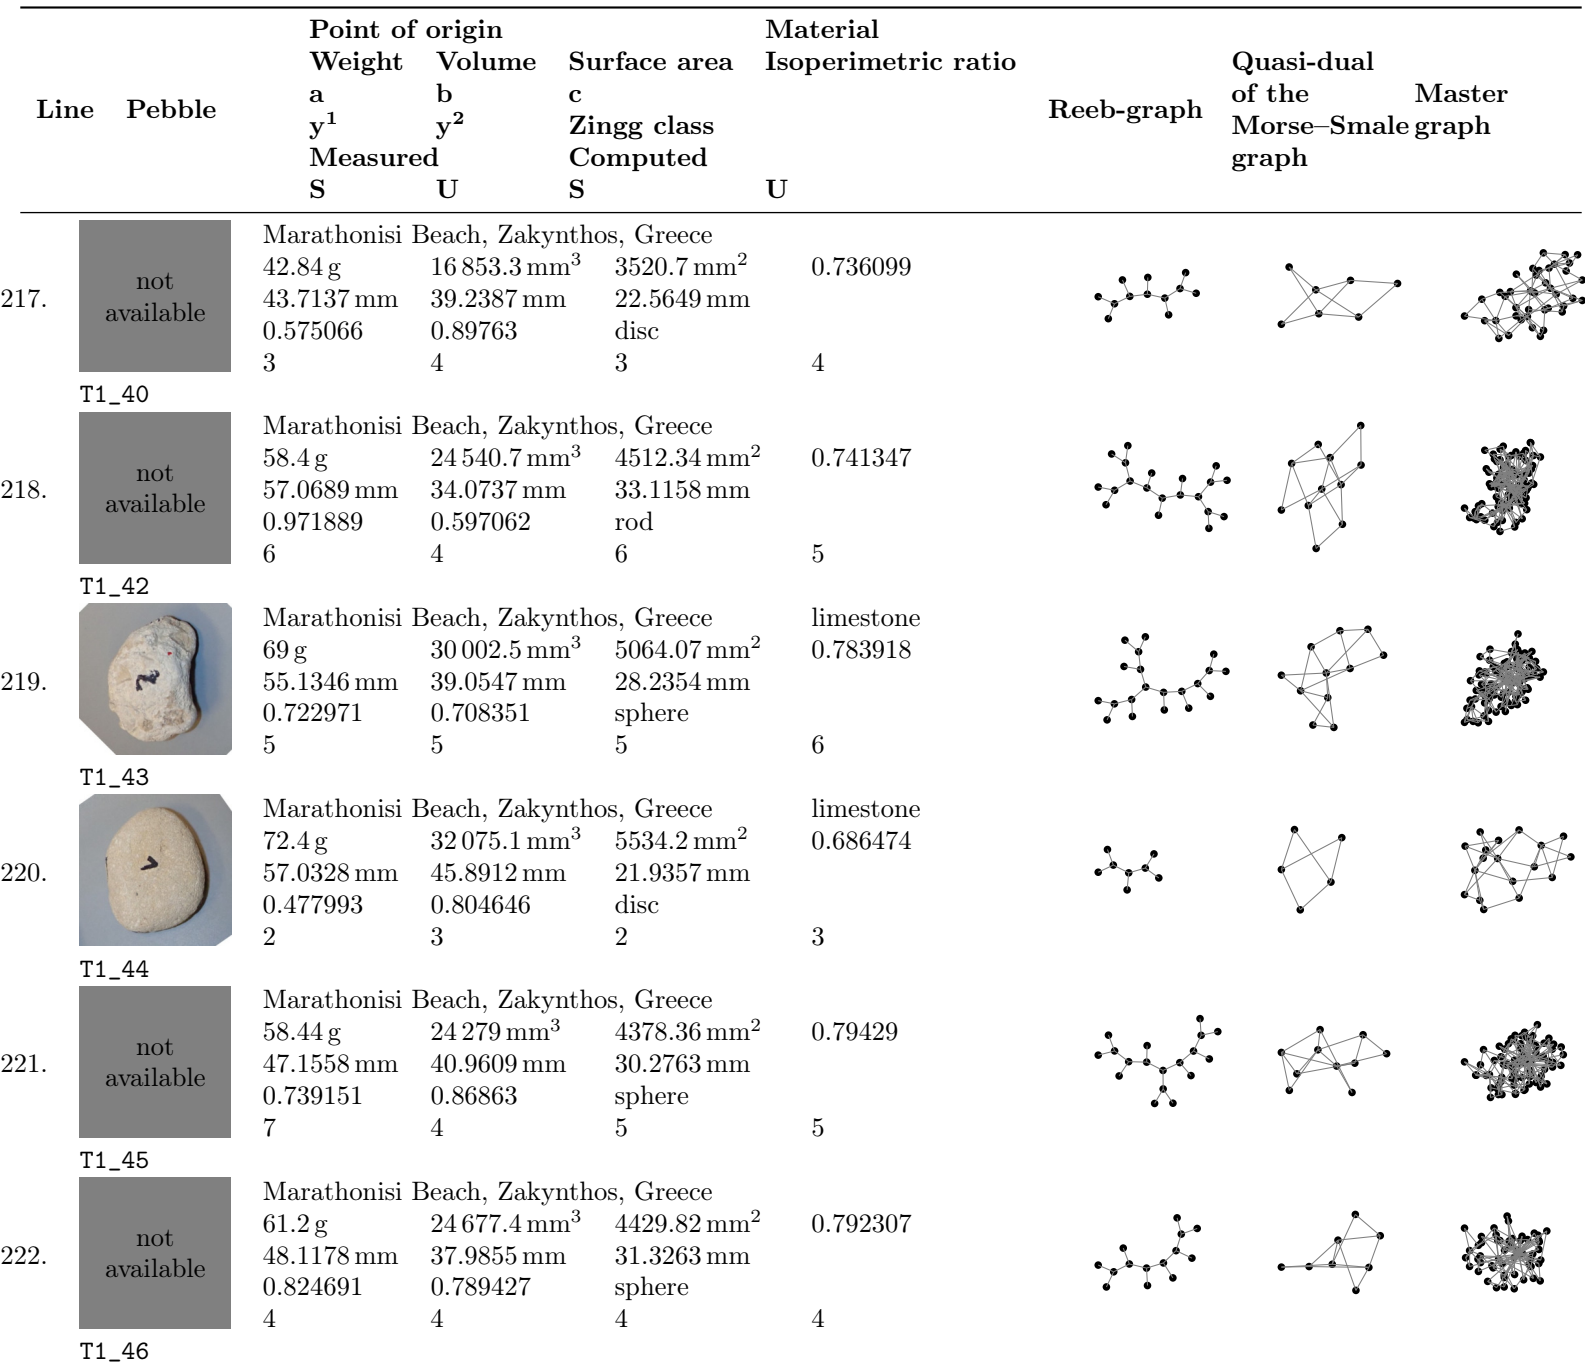 |
|      | T1_46                                                                               |                                                                                |                                                         |                                                      |                                      |                                                                                       |                                                                                       |                                                                                       |

| Line | Pebble                                                                              | Point of origin                                                                |                                                                    | Surface area<br>c<br>Zingg class<br>Computed<br>S    | Material<br>Isoperimetric ratio<br>U | Reeb-graph                                                                            | Quasi-dual<br>of the<br>Morse–Smale<br>graph                                          | Master<br>graph                                                                       |
|------|-------------------------------------------------------------------------------------|--------------------------------------------------------------------------------|--------------------------------------------------------------------|------------------------------------------------------|--------------------------------------|---------------------------------------------------------------------------------------|---------------------------------------------------------------------------------------|---------------------------------------------------------------------------------------|
|      |                                                                                     | Weight                                                                         | Volume                                                             |                                                      |                                      |                                                                                       |                                                                                       |                                                                                       |
|      |                                                                                     | a<br>y <sup>1</sup><br>Measured<br>S                                           | b<br>y <sup>2</sup><br>U                                           |                                                      |                                      |                                                                                       |                                                                                       |                                                                                       |
|      |                                                                                     |                                                                                |                                                                    |                                                      |                                      |                                                                                       |                                                                                       |                                                                                       |
| 223. | 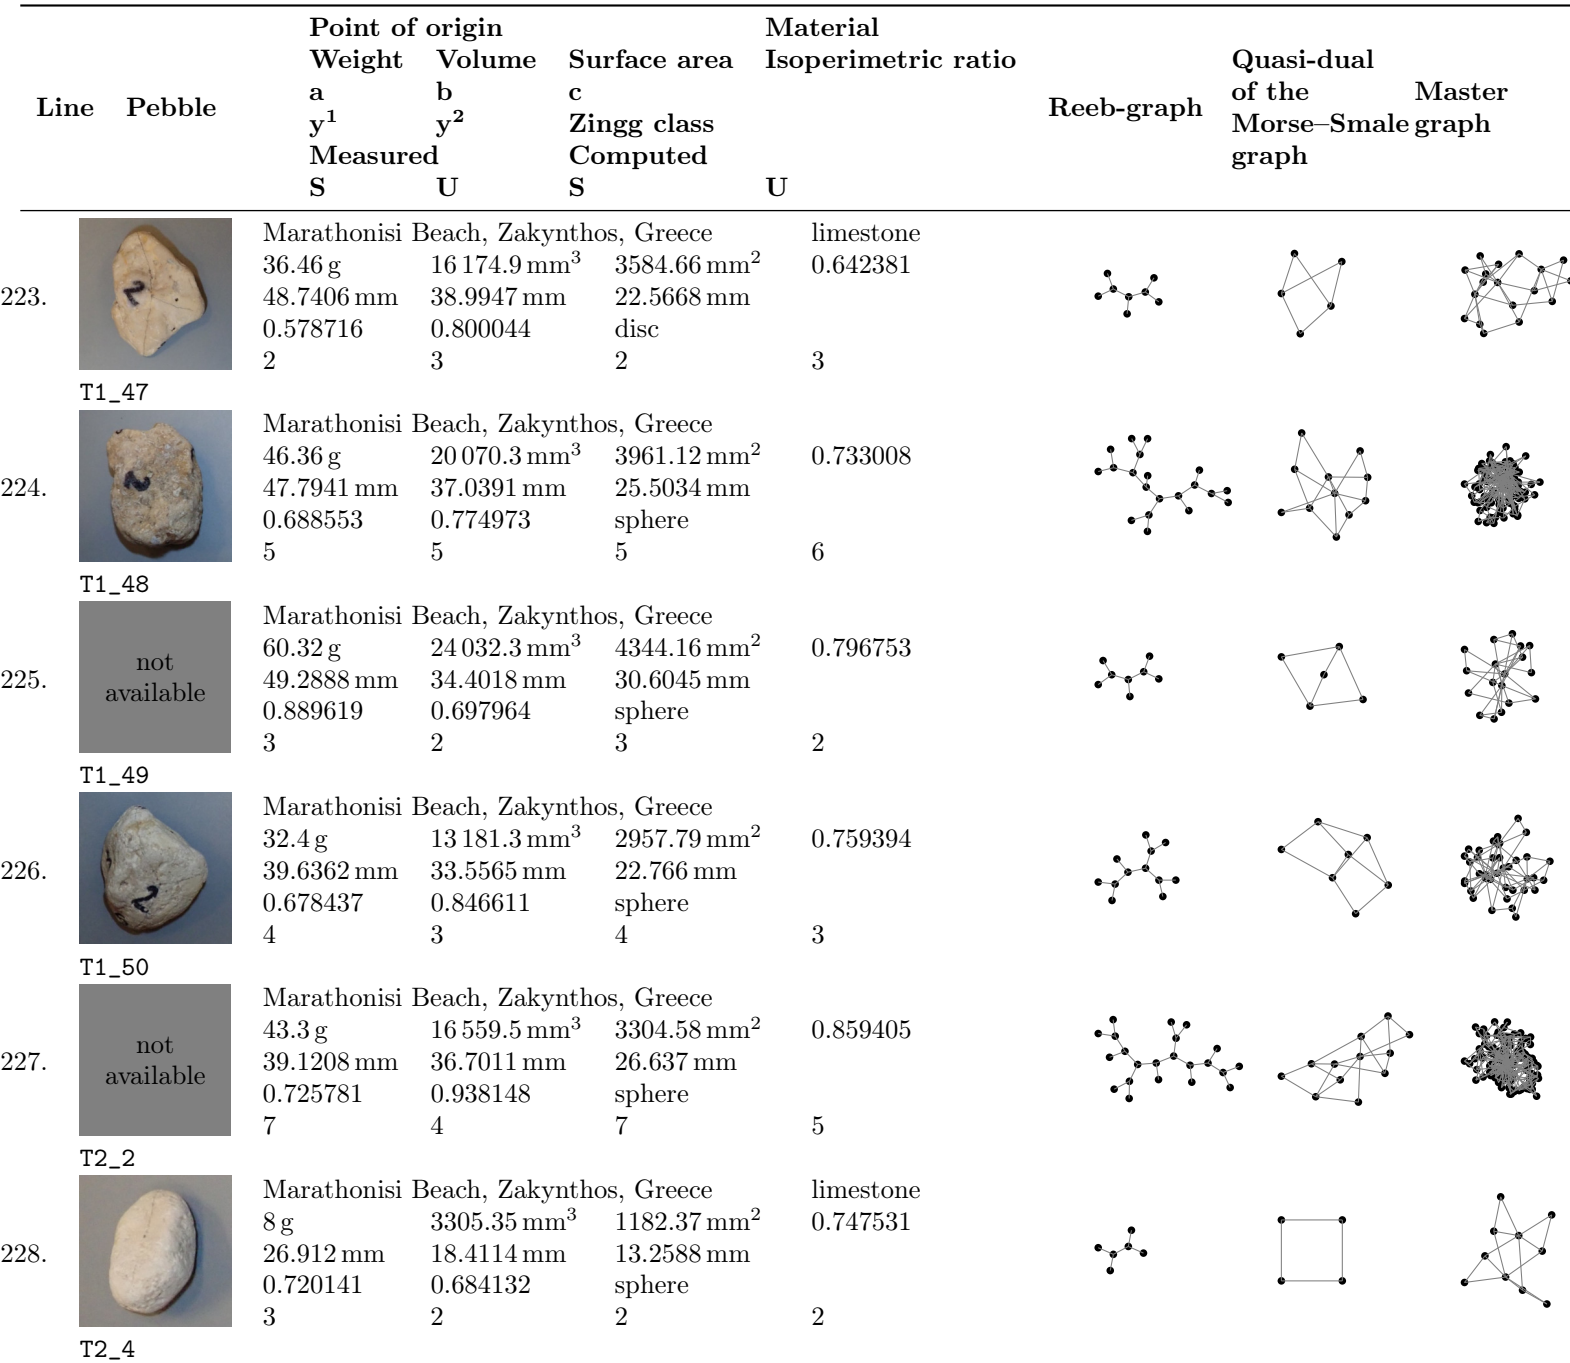   | Marathonisi Beach, Zakynthos, Greece<br>36.46 g<br>48.7406 mm<br>0.578716<br>2 | 36.46 g<br>16 174.9 mm <sup>3</sup><br>38.9947 mm<br>0.800044<br>3 | 3584.66 mm <sup>2</sup><br>22.5668 mm<br>disc<br>2   | limestone<br>0.642381<br>3           | 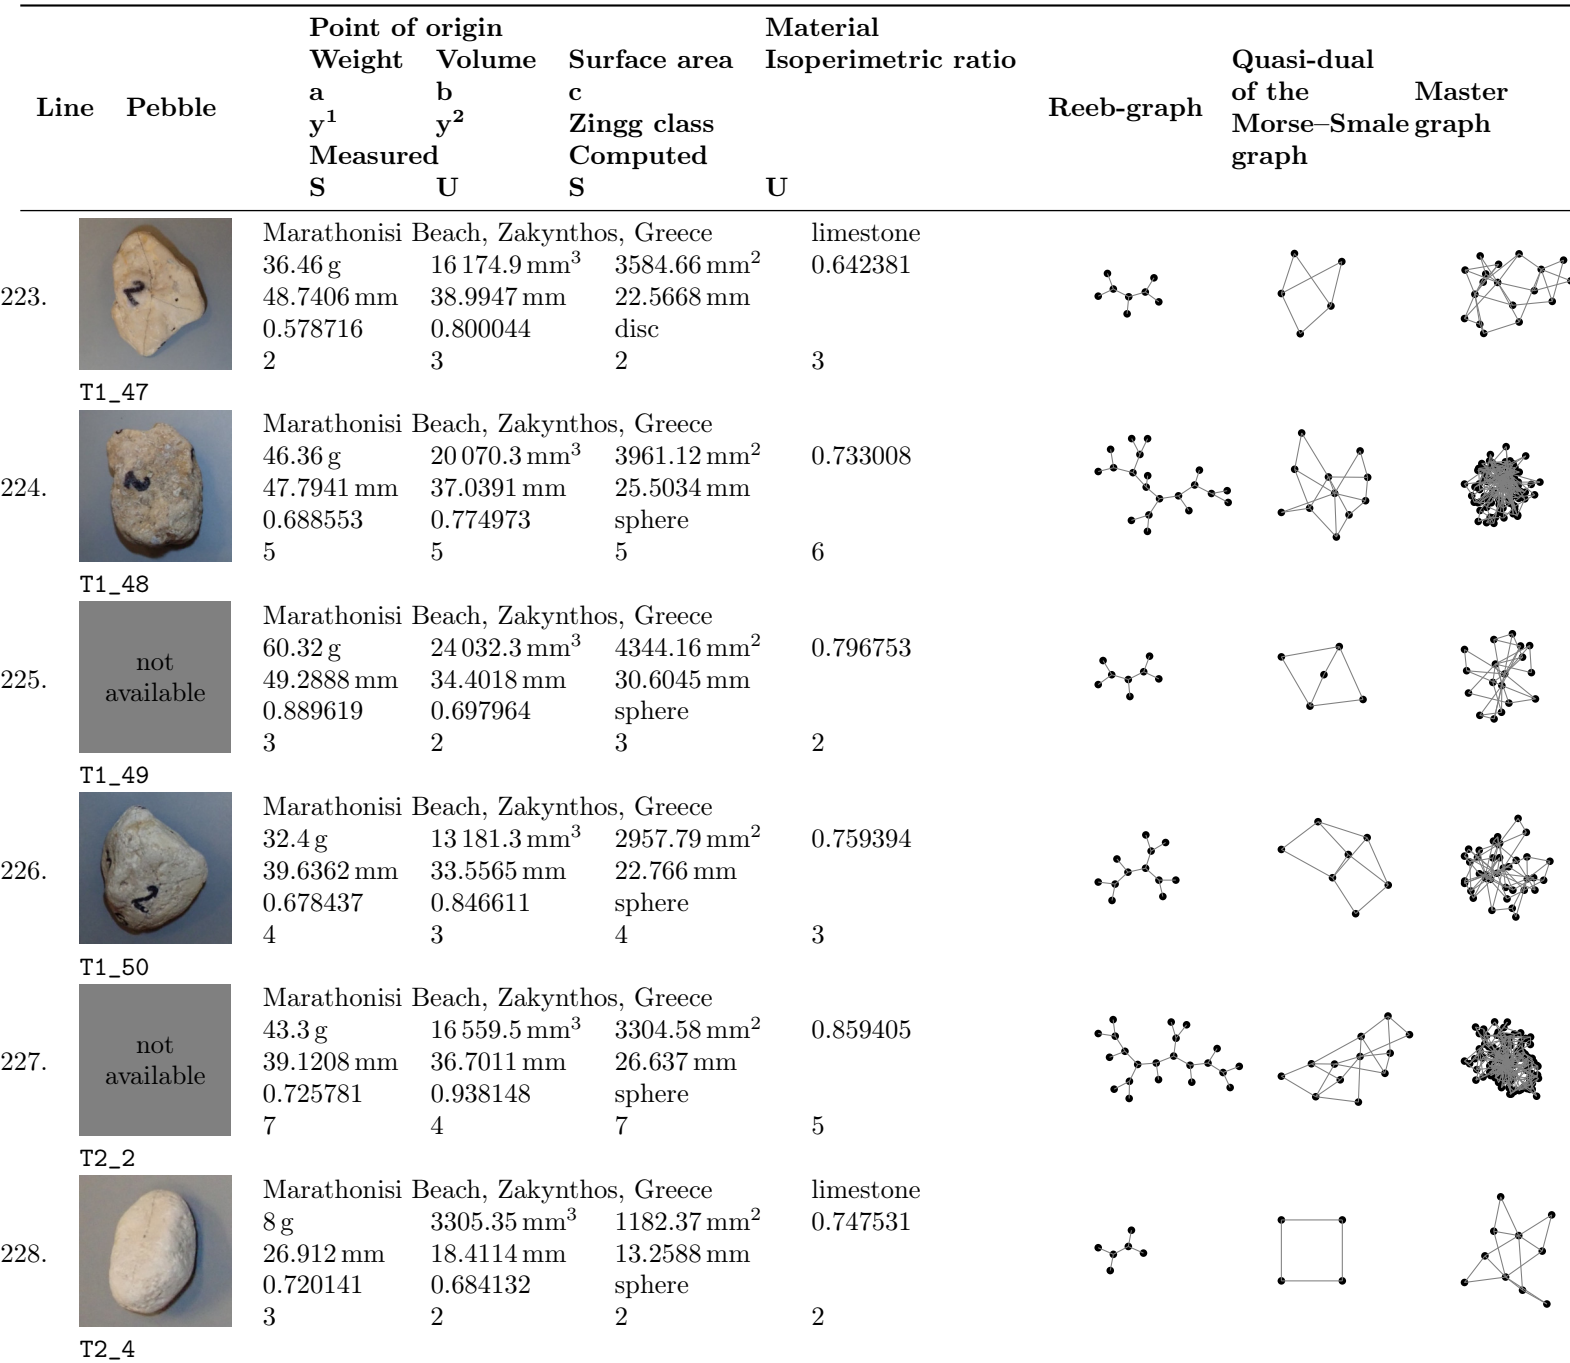   | 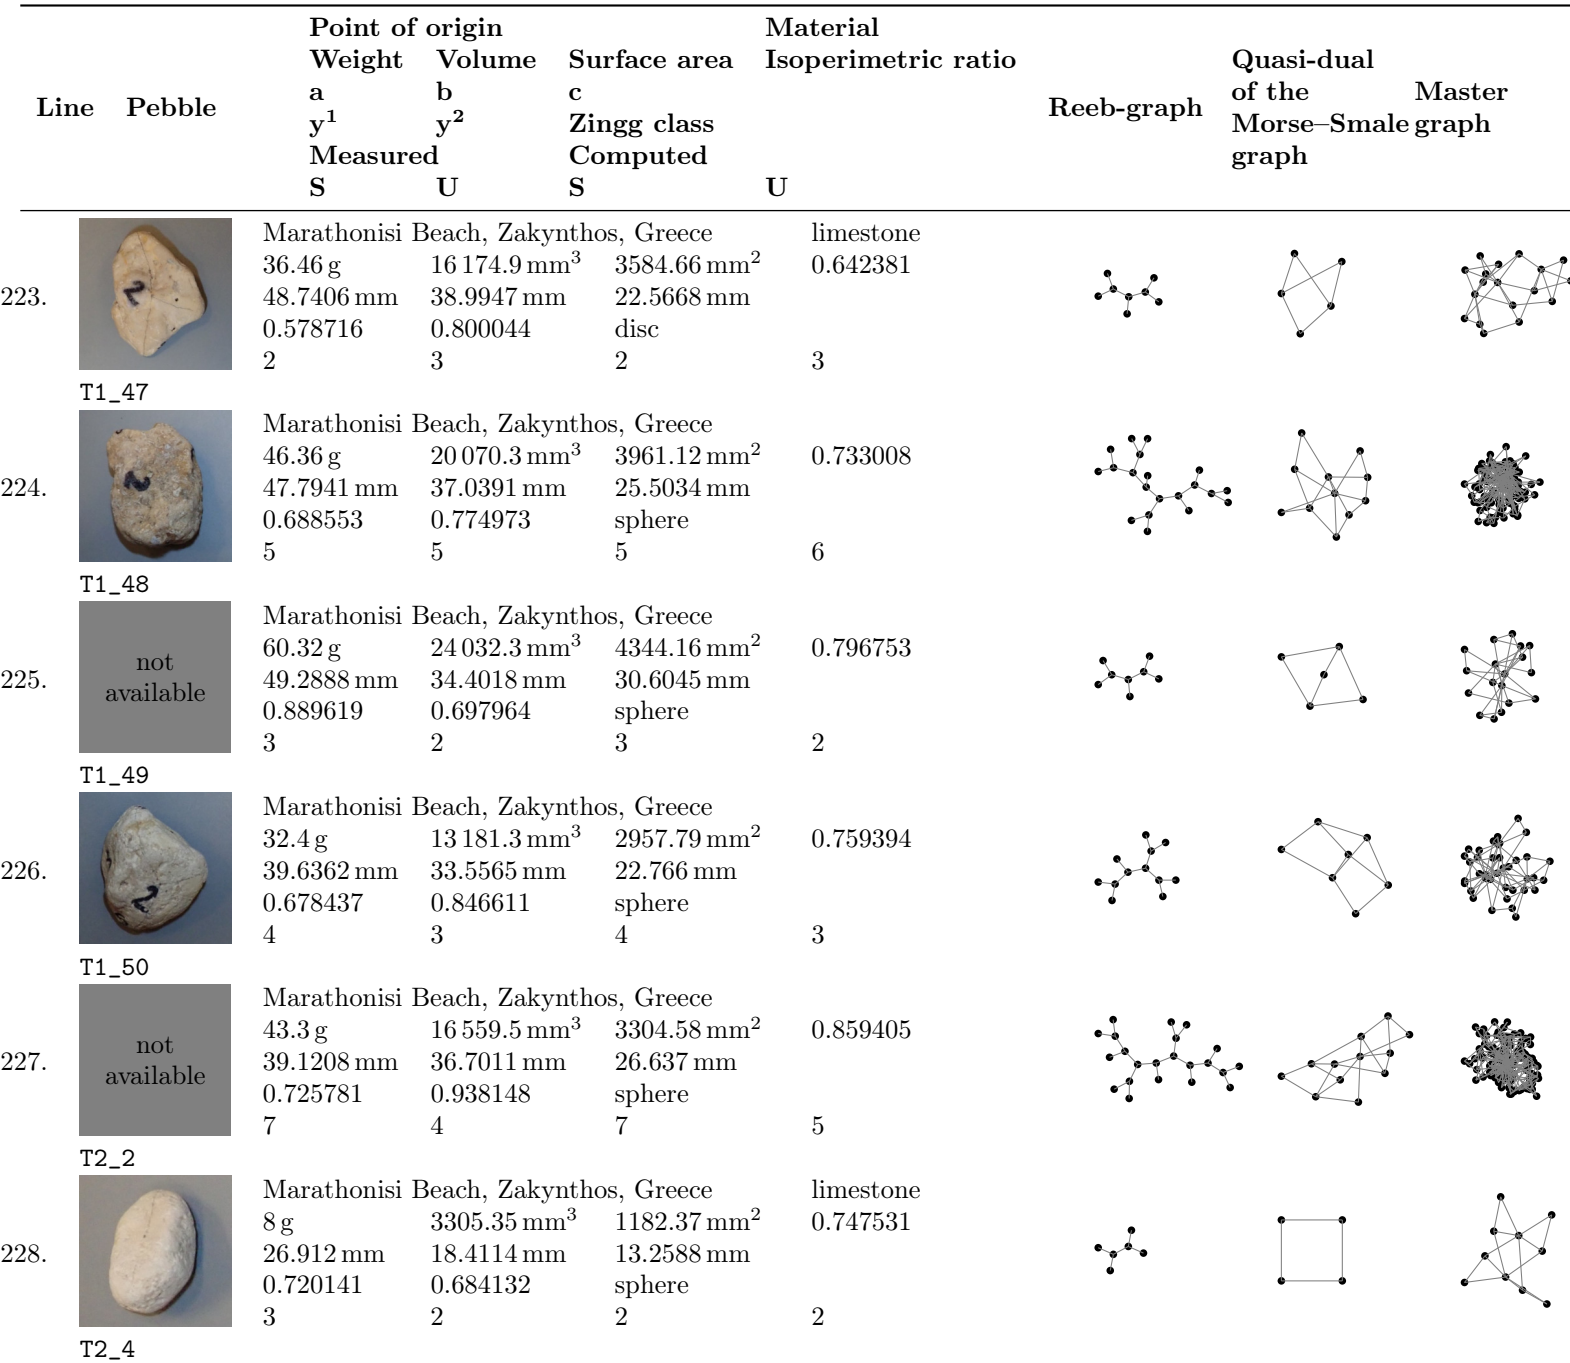   | 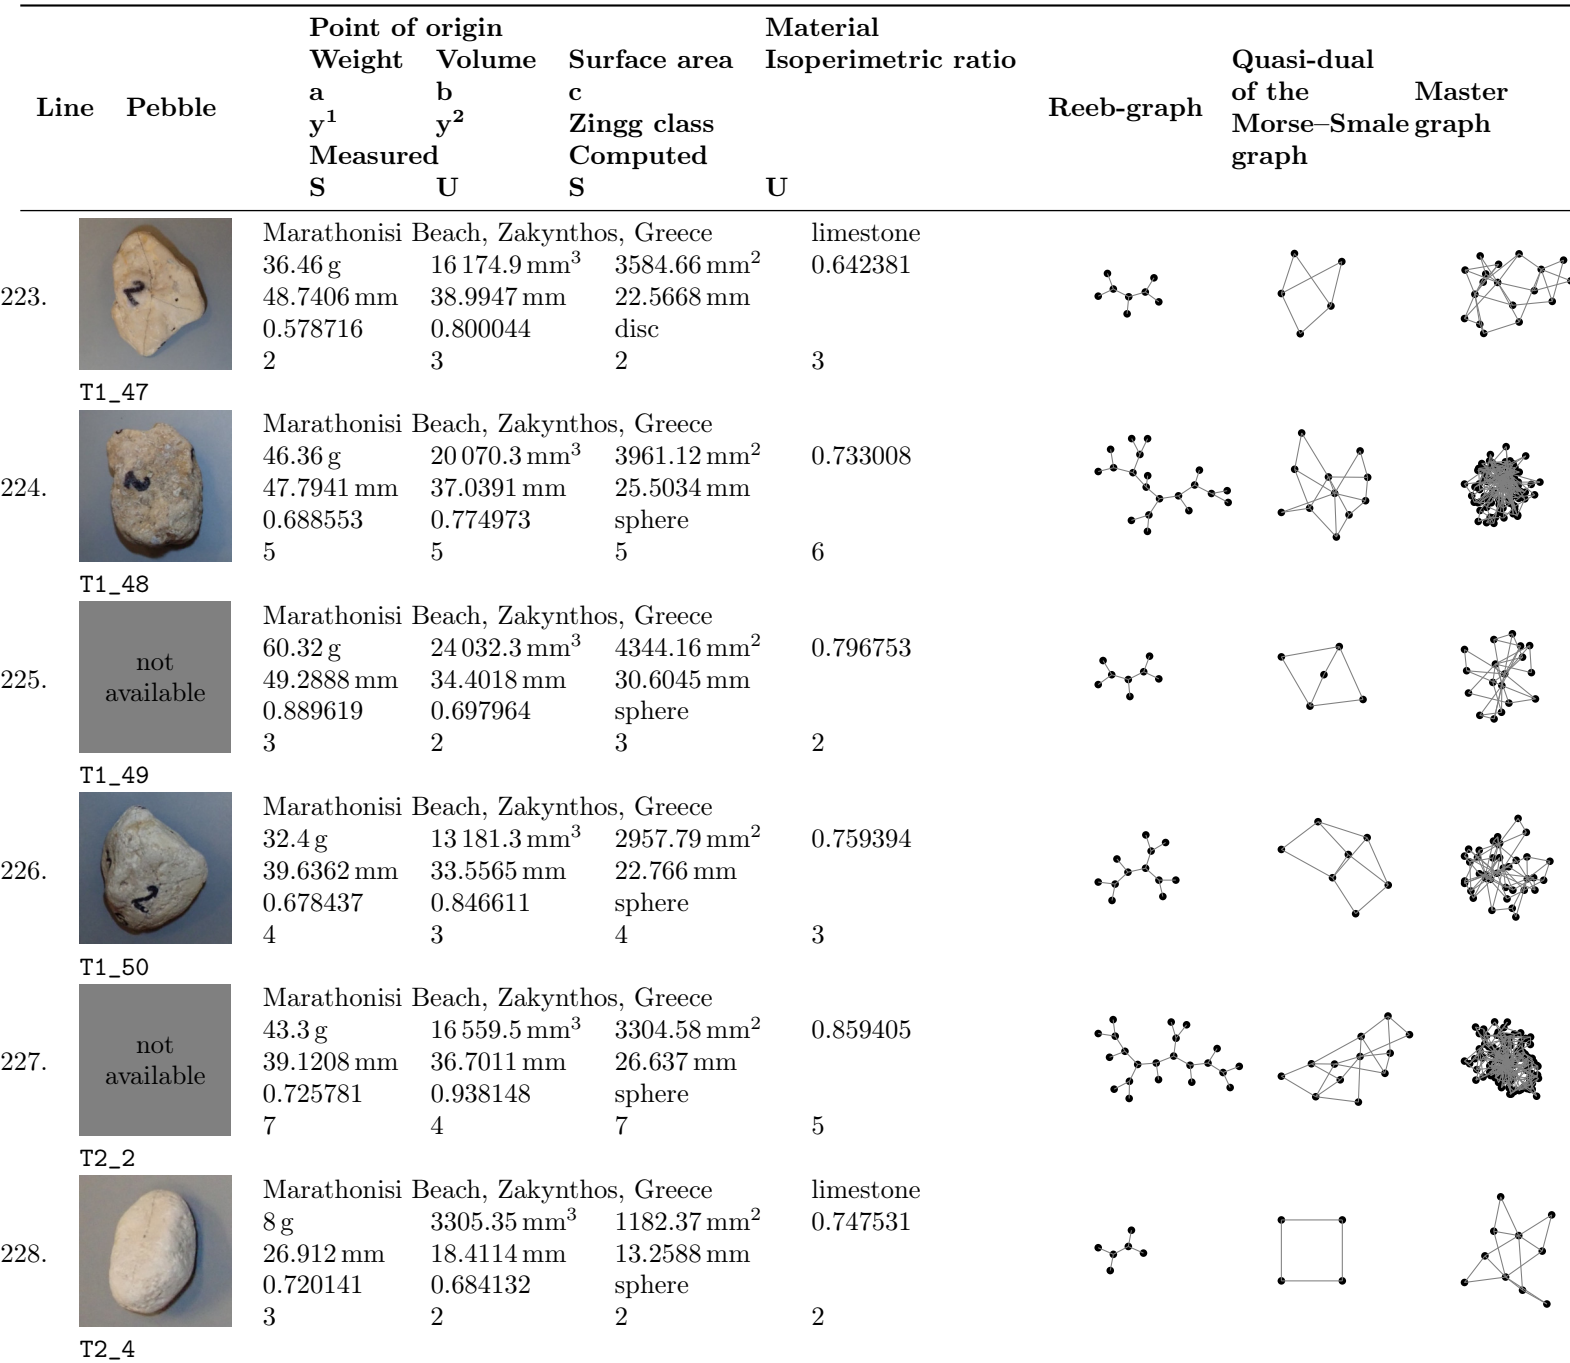   |
|      | T1_47                                                                               |                                                                                |                                                                    |                                                      |                                      |                                                                                       |                                                                                       |                                                                                       |
| 224. | 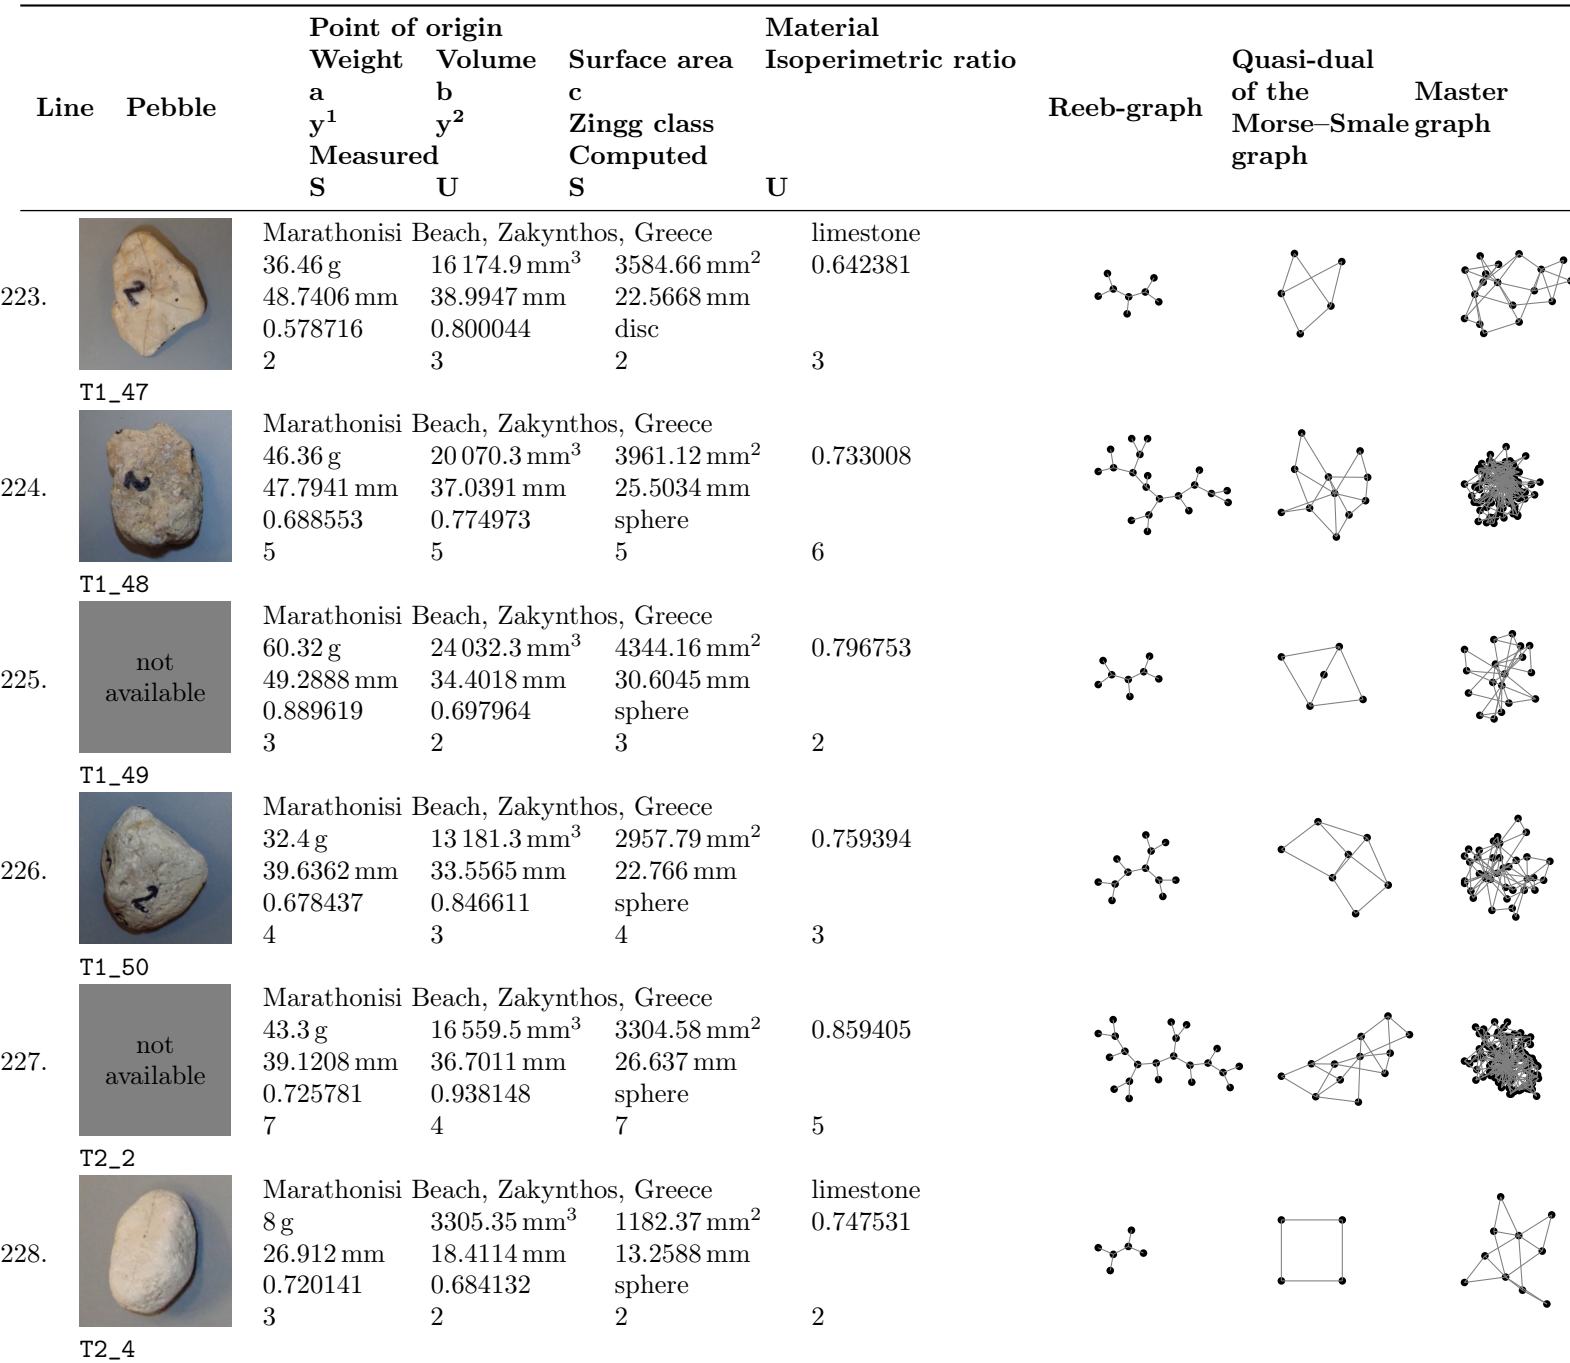   | Marathonisi Beach, Zakynthos, Greece<br>46.36 g<br>47.7941 mm<br>0.688553<br>5 | 46.36 g<br>20 070.3 mm <sup>3</sup><br>37.0391 mm<br>0.774973<br>5 | 3961.12 mm <sup>2</sup><br>25.5034 mm<br>sphere<br>5 | 0.733008<br>6                        | 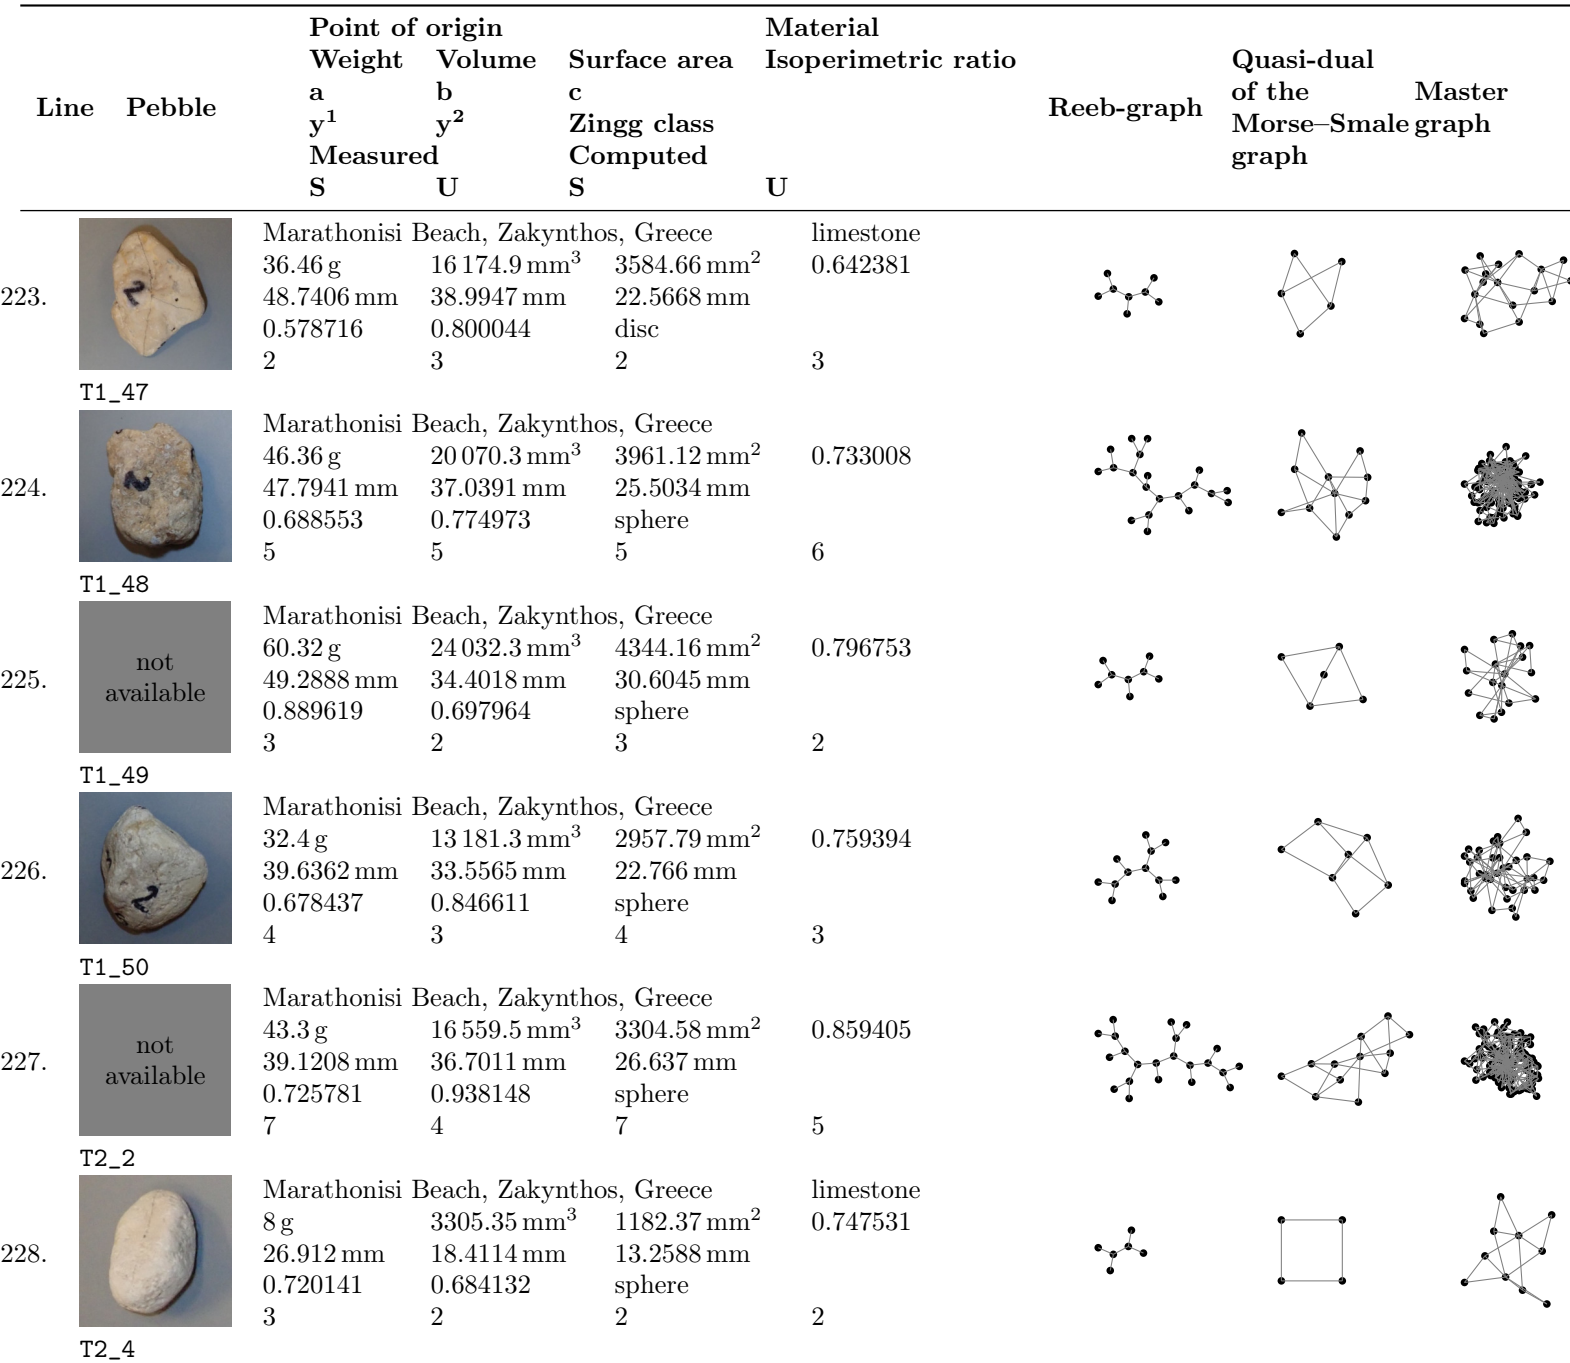   | 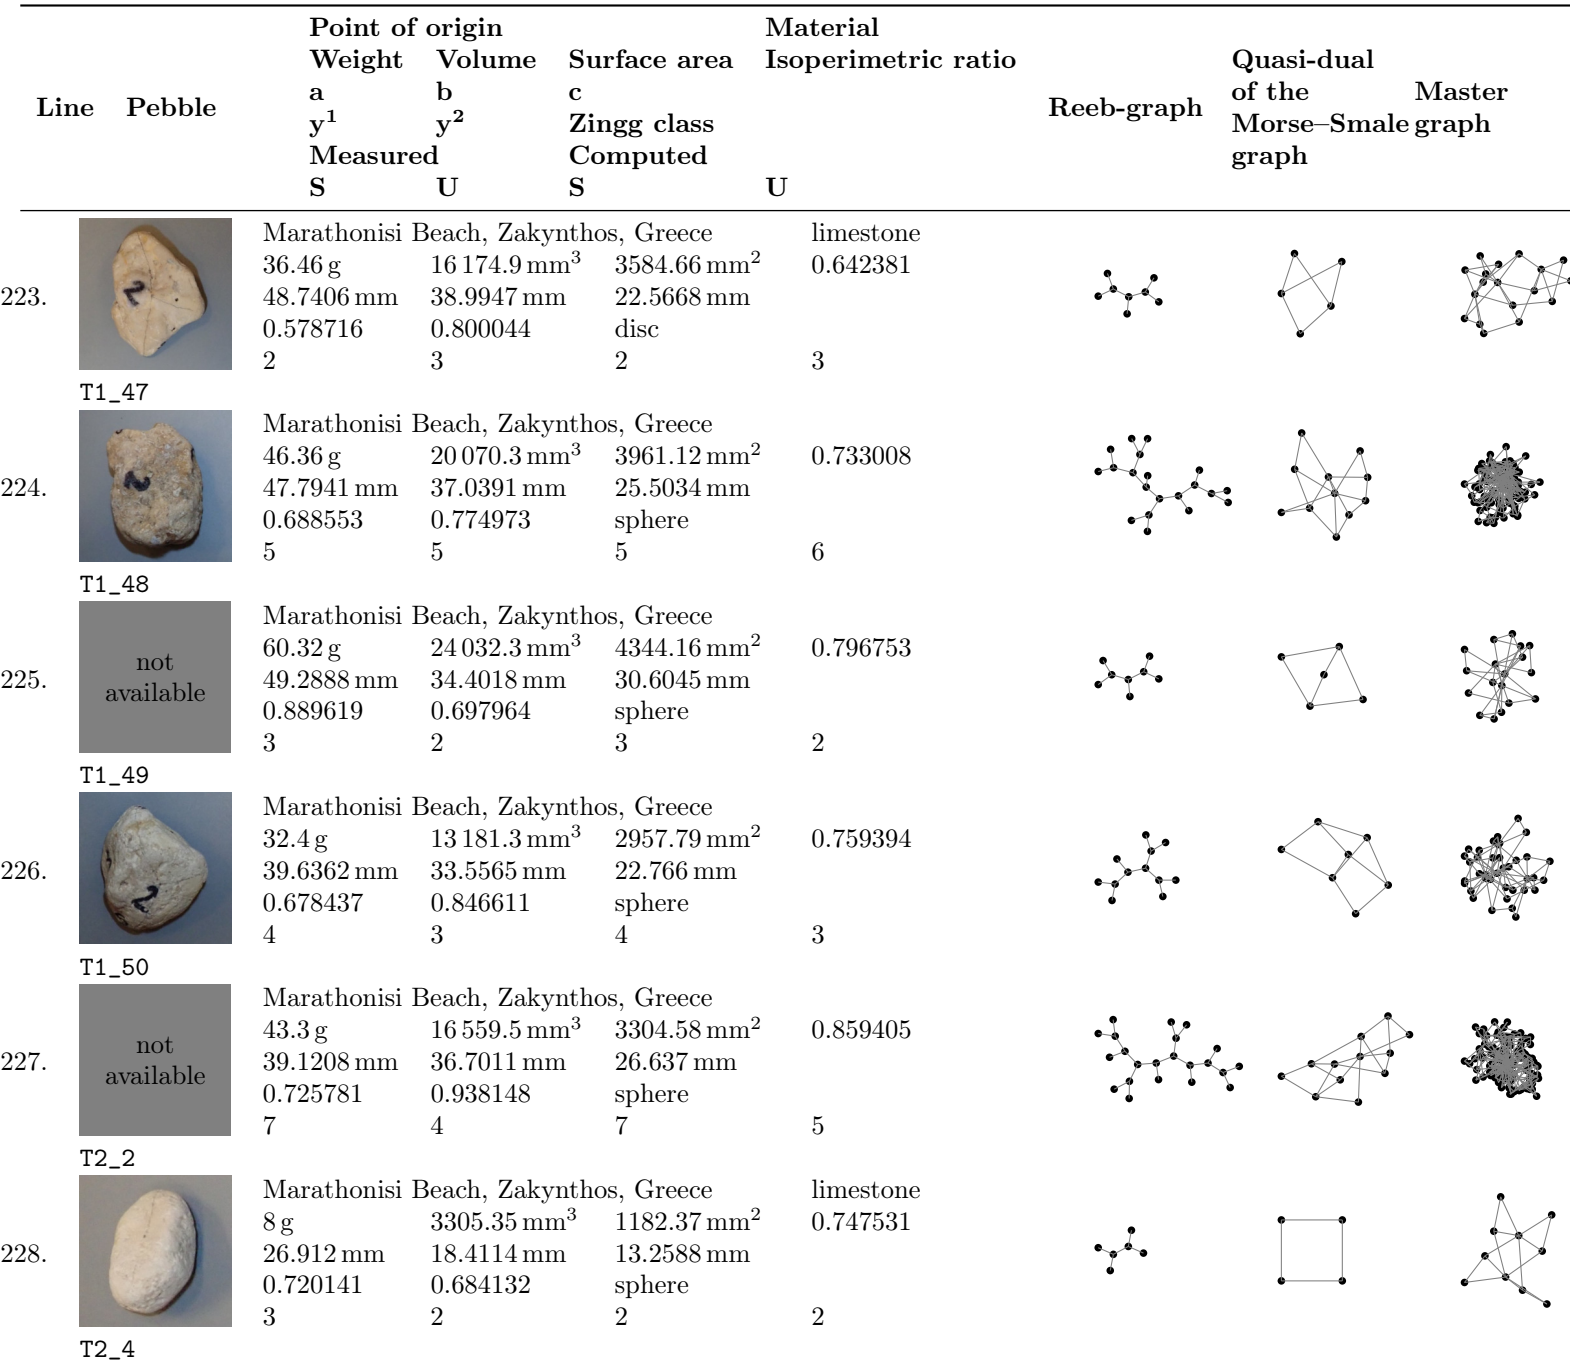   | 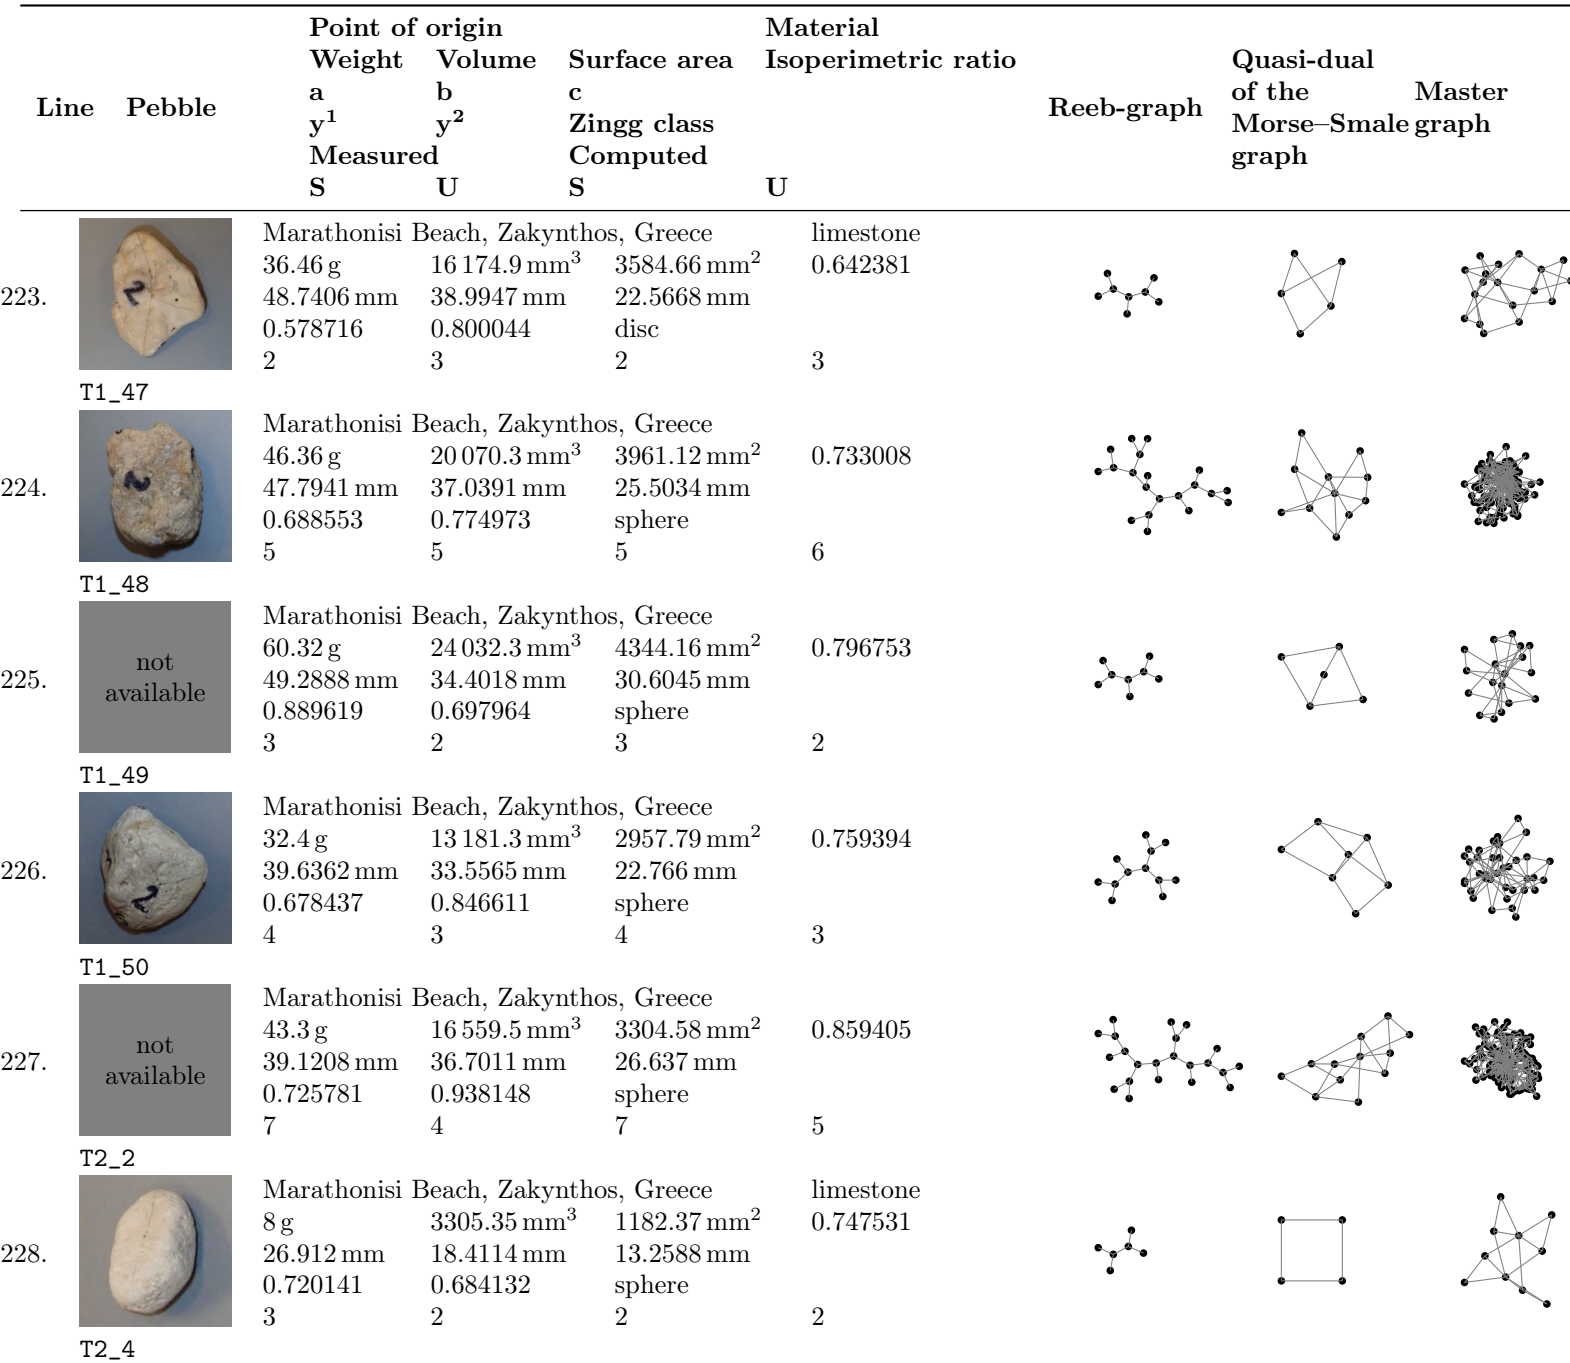   |
|      | T1_48                                                                               |                                                                                |                                                                    |                                                      |                                      |                                                                                       |                                                                                       |                                                                                       |
| 225. | 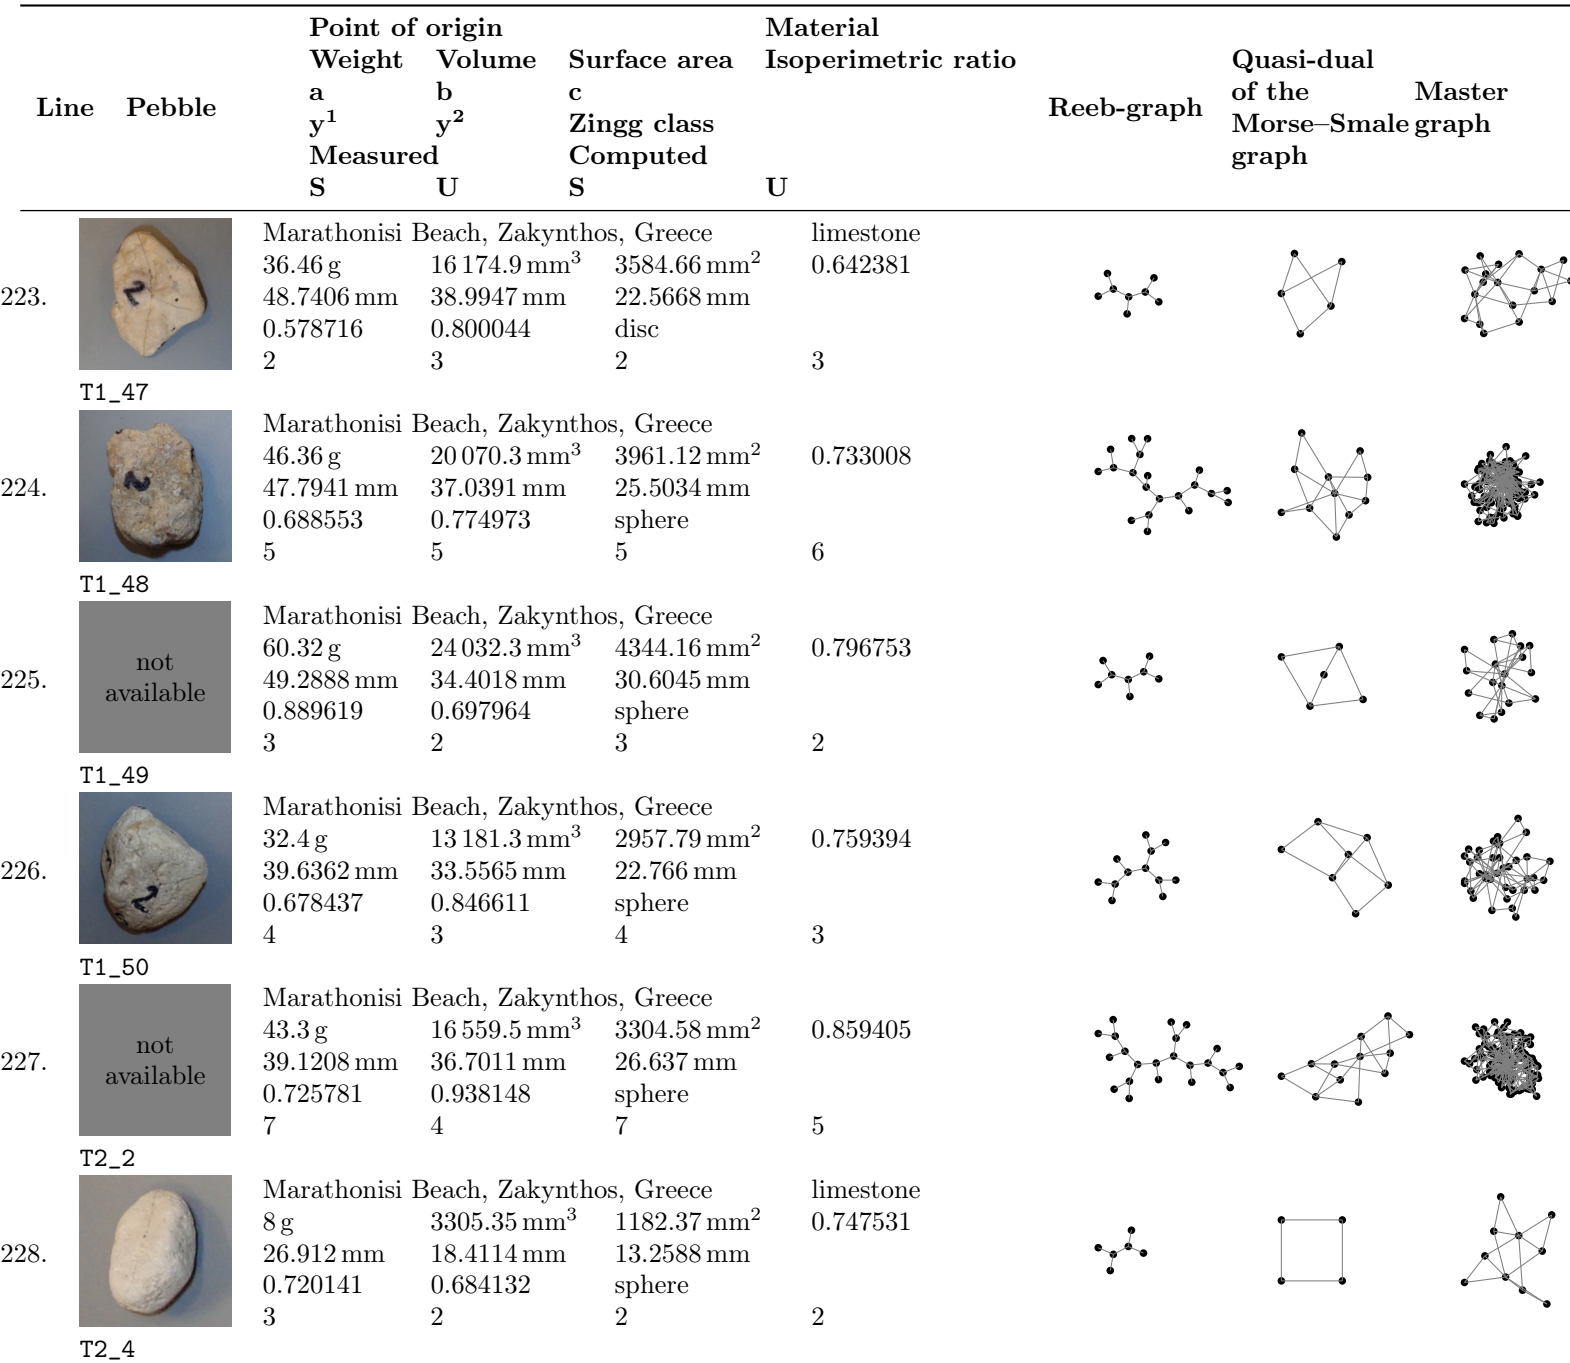   | Marathonisi Beach, Zakynthos, Greece<br>60.32 g<br>49.2888 mm<br>0.889619<br>3 | 60.32 g<br>24 032.3 mm <sup>3</sup><br>34.4018 mm<br>0.697964<br>2 | 4344.16 mm <sup>2</sup><br>30.6045 mm<br>sphere<br>3 | 0.796753<br>2                        | 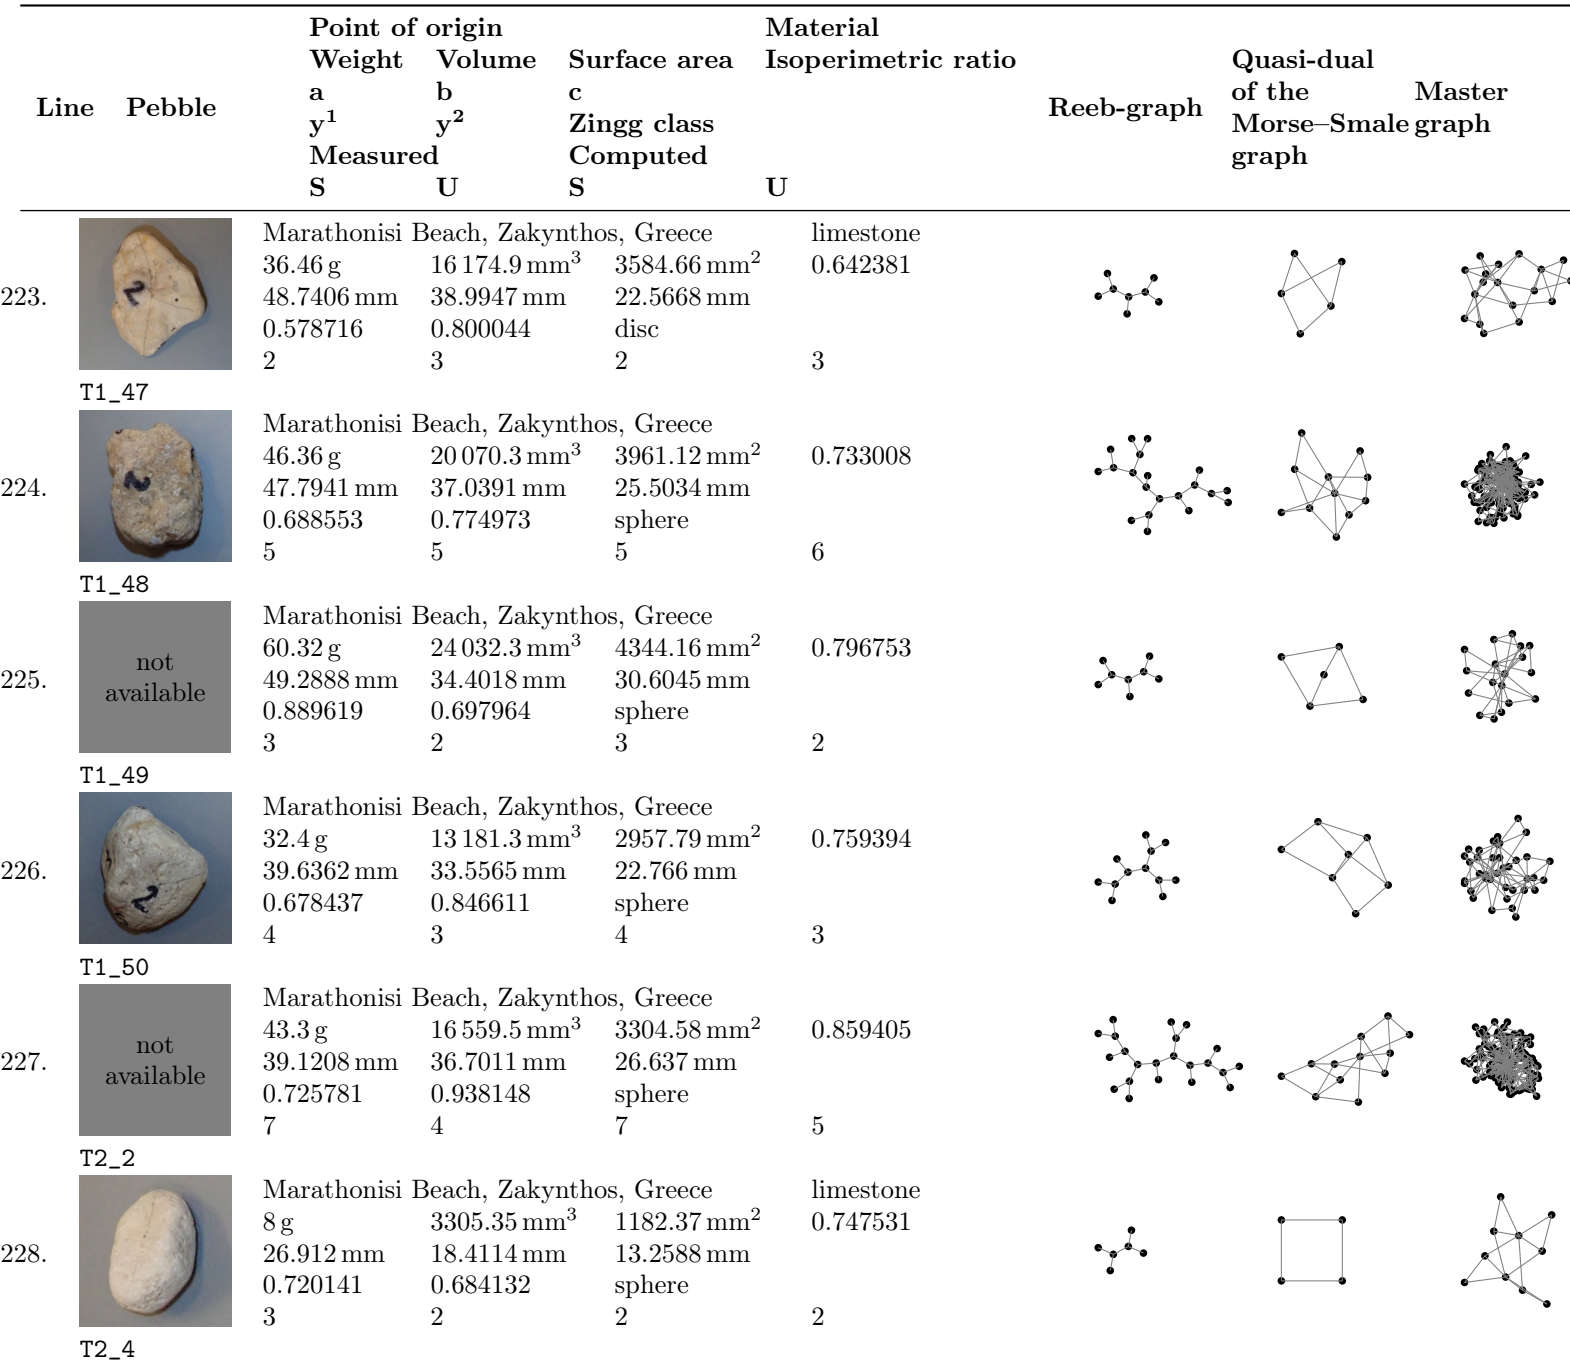   | 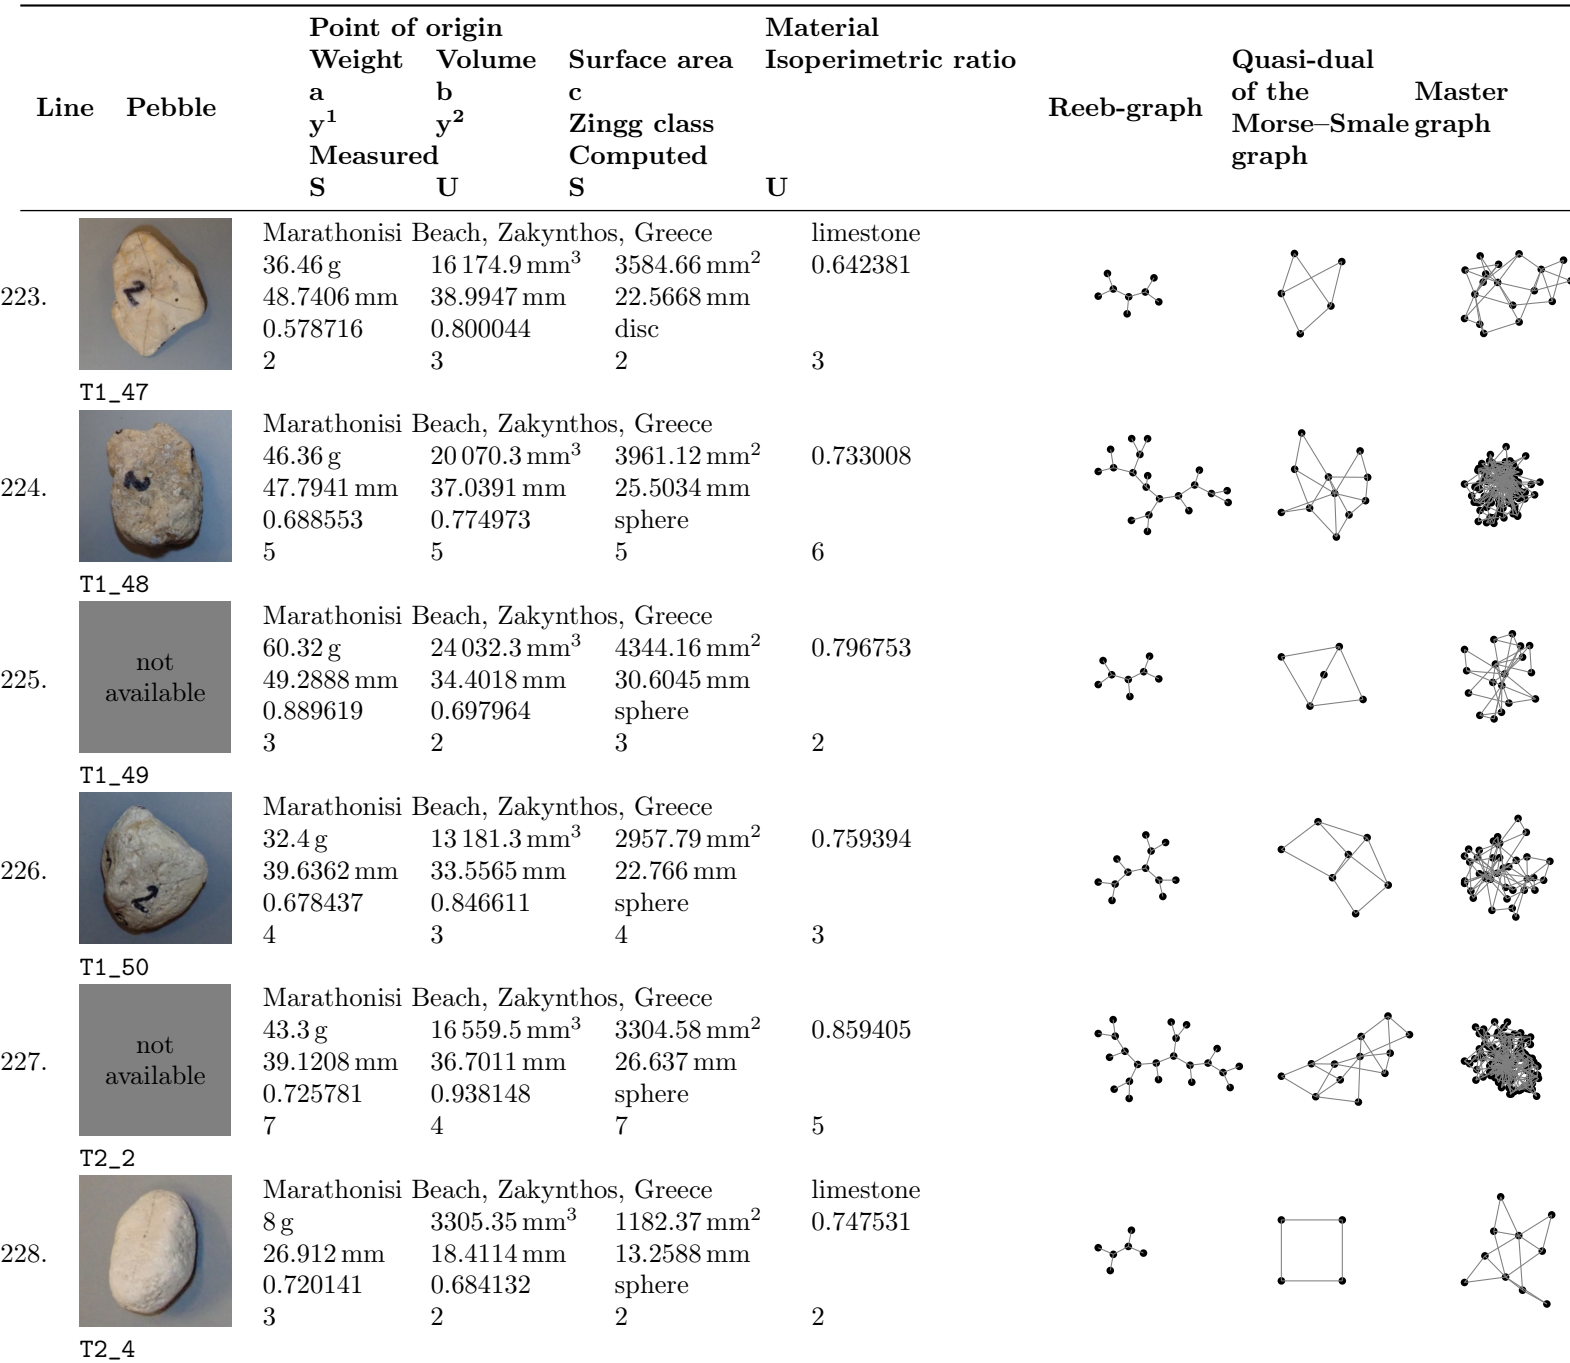   | 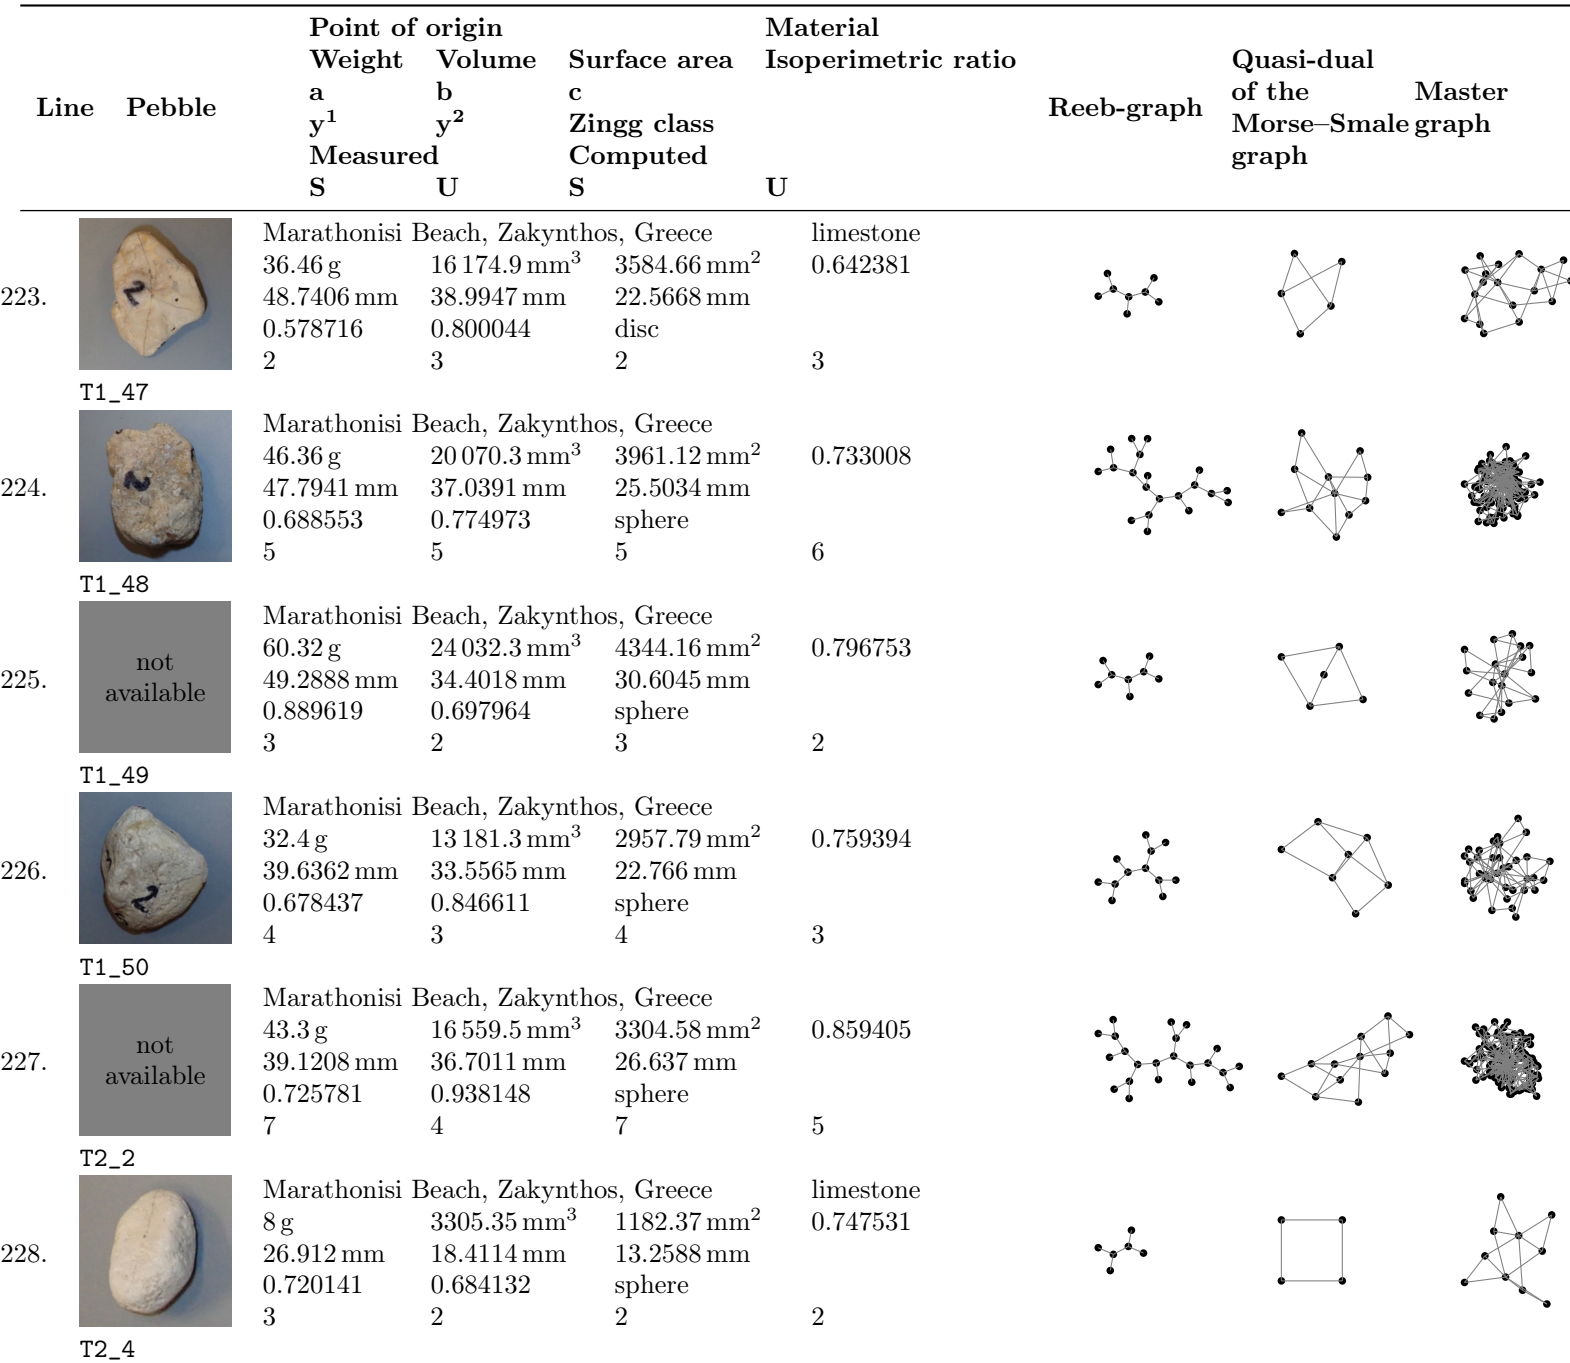   |
|      | T1_49                                                                               |                                                                                |                                                                    |                                                      |                                      |                                                                                       |                                                                                       |                                                                                       |
| 226. | 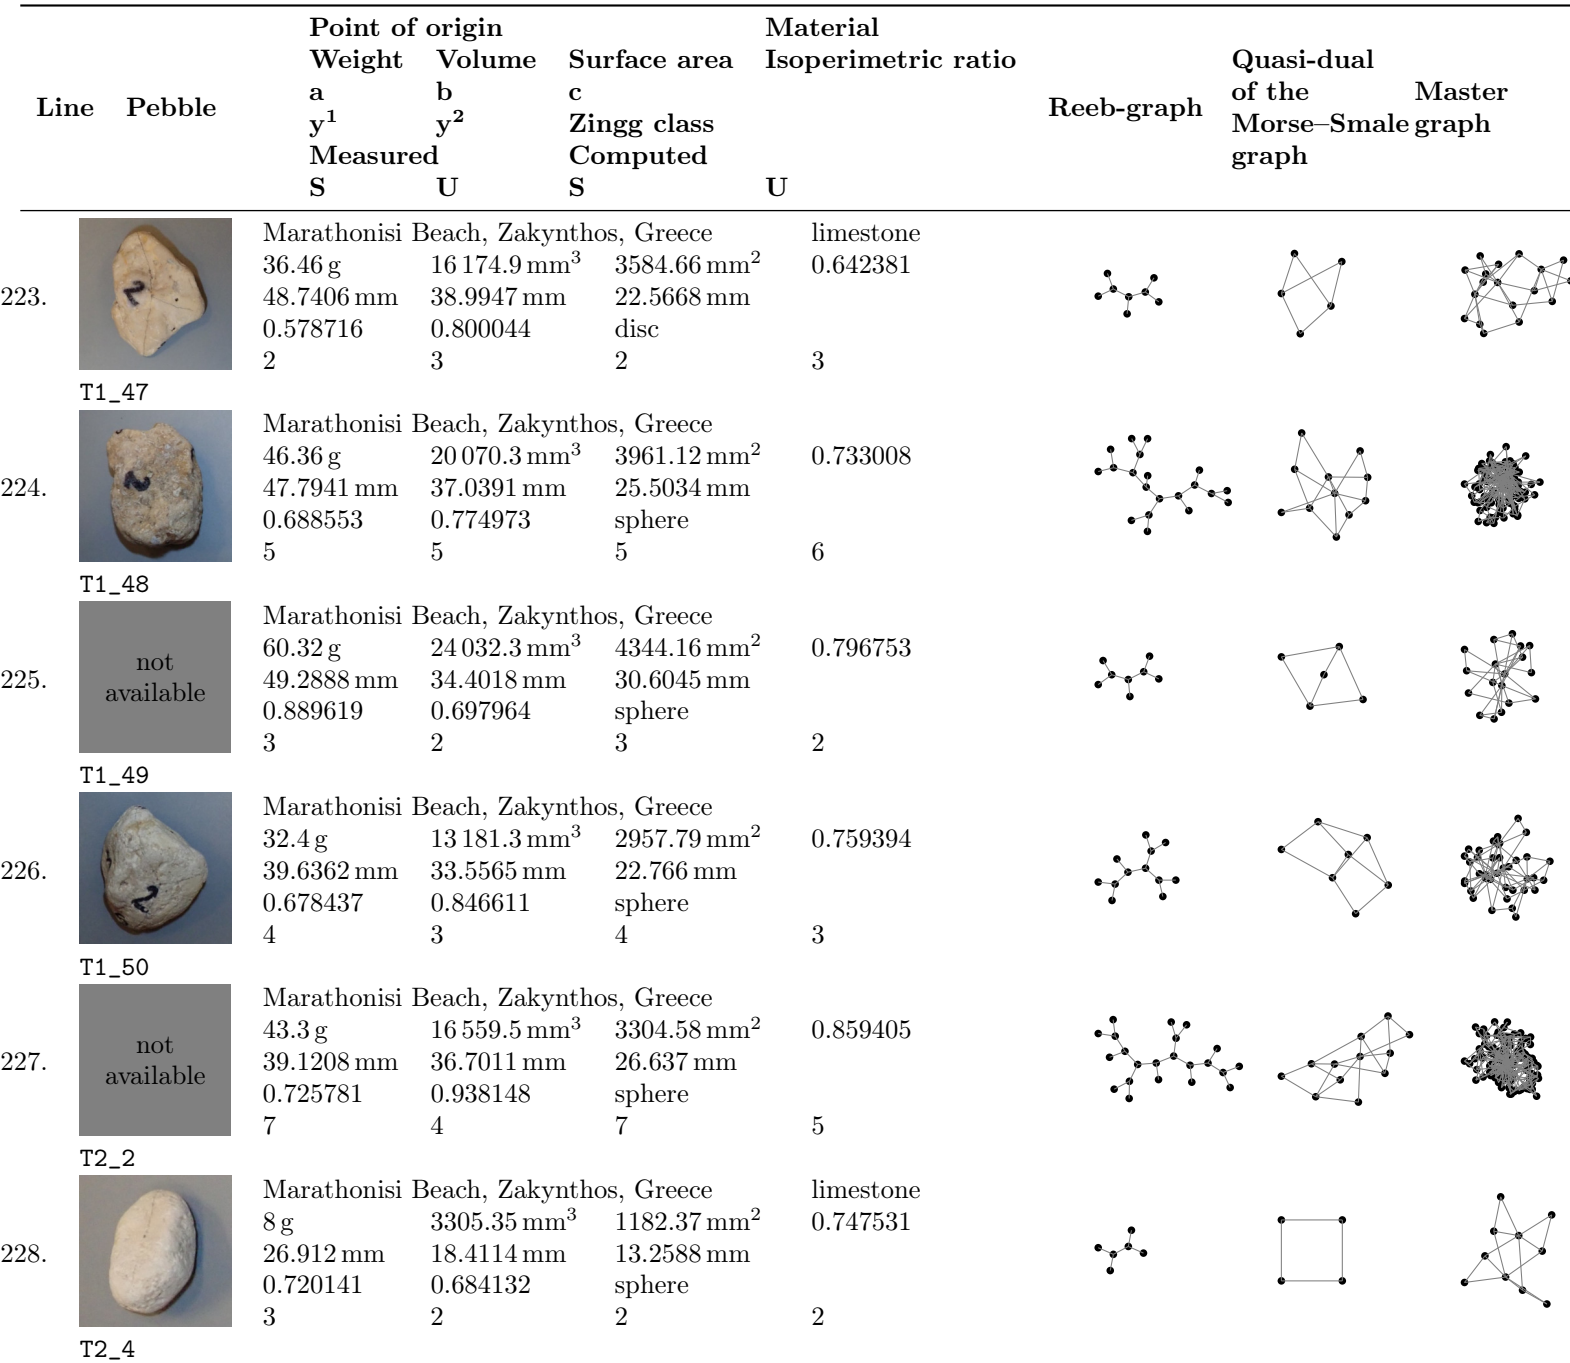  | Marathonisi Beach, Zakynthos, Greece<br>32.4 g<br>39.6362 mm<br>0.678437<br>4  | 32.4 g<br>13 181.3 mm <sup>3</sup><br>33.5565 mm<br>0.846611<br>3  | 2957.79 mm <sup>2</sup><br>22.766 mm<br>sphere<br>4  | 0.759394<br>3                        | 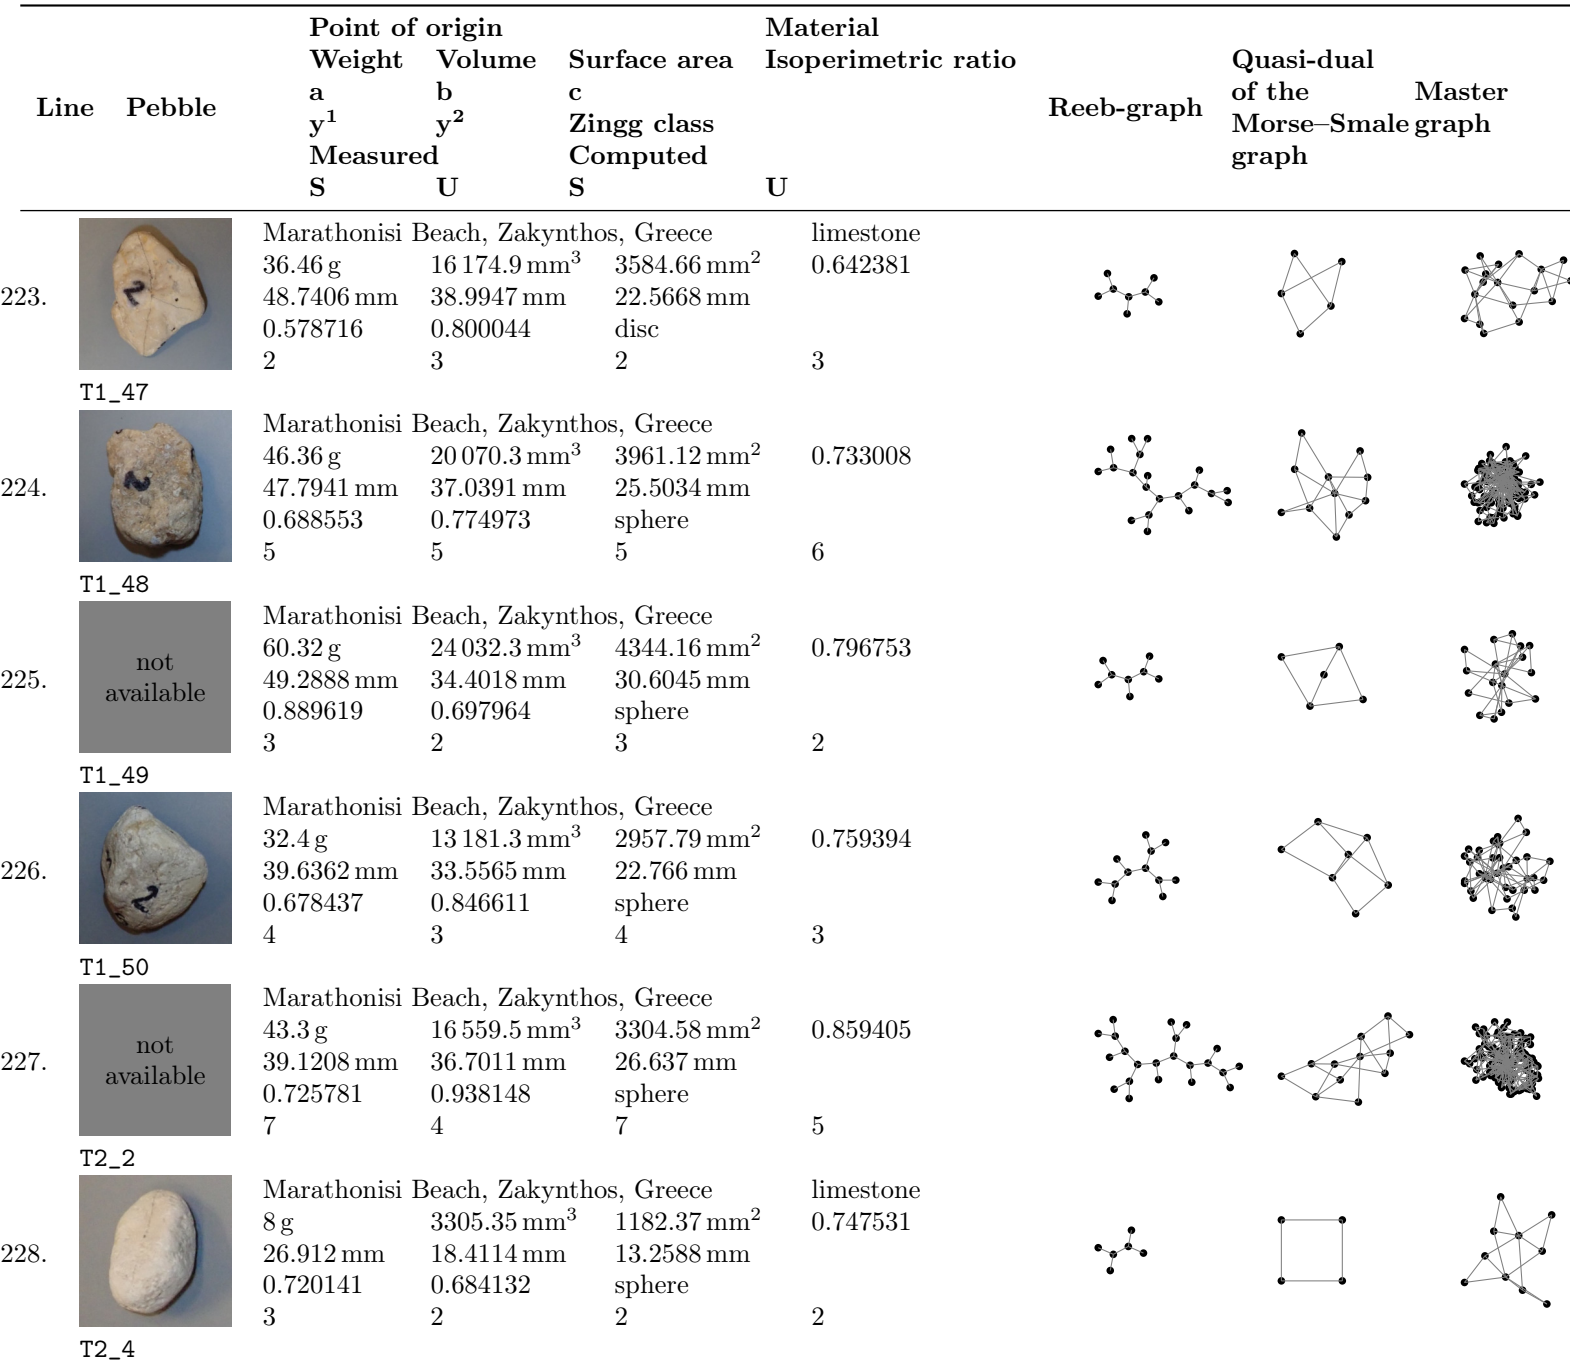  | 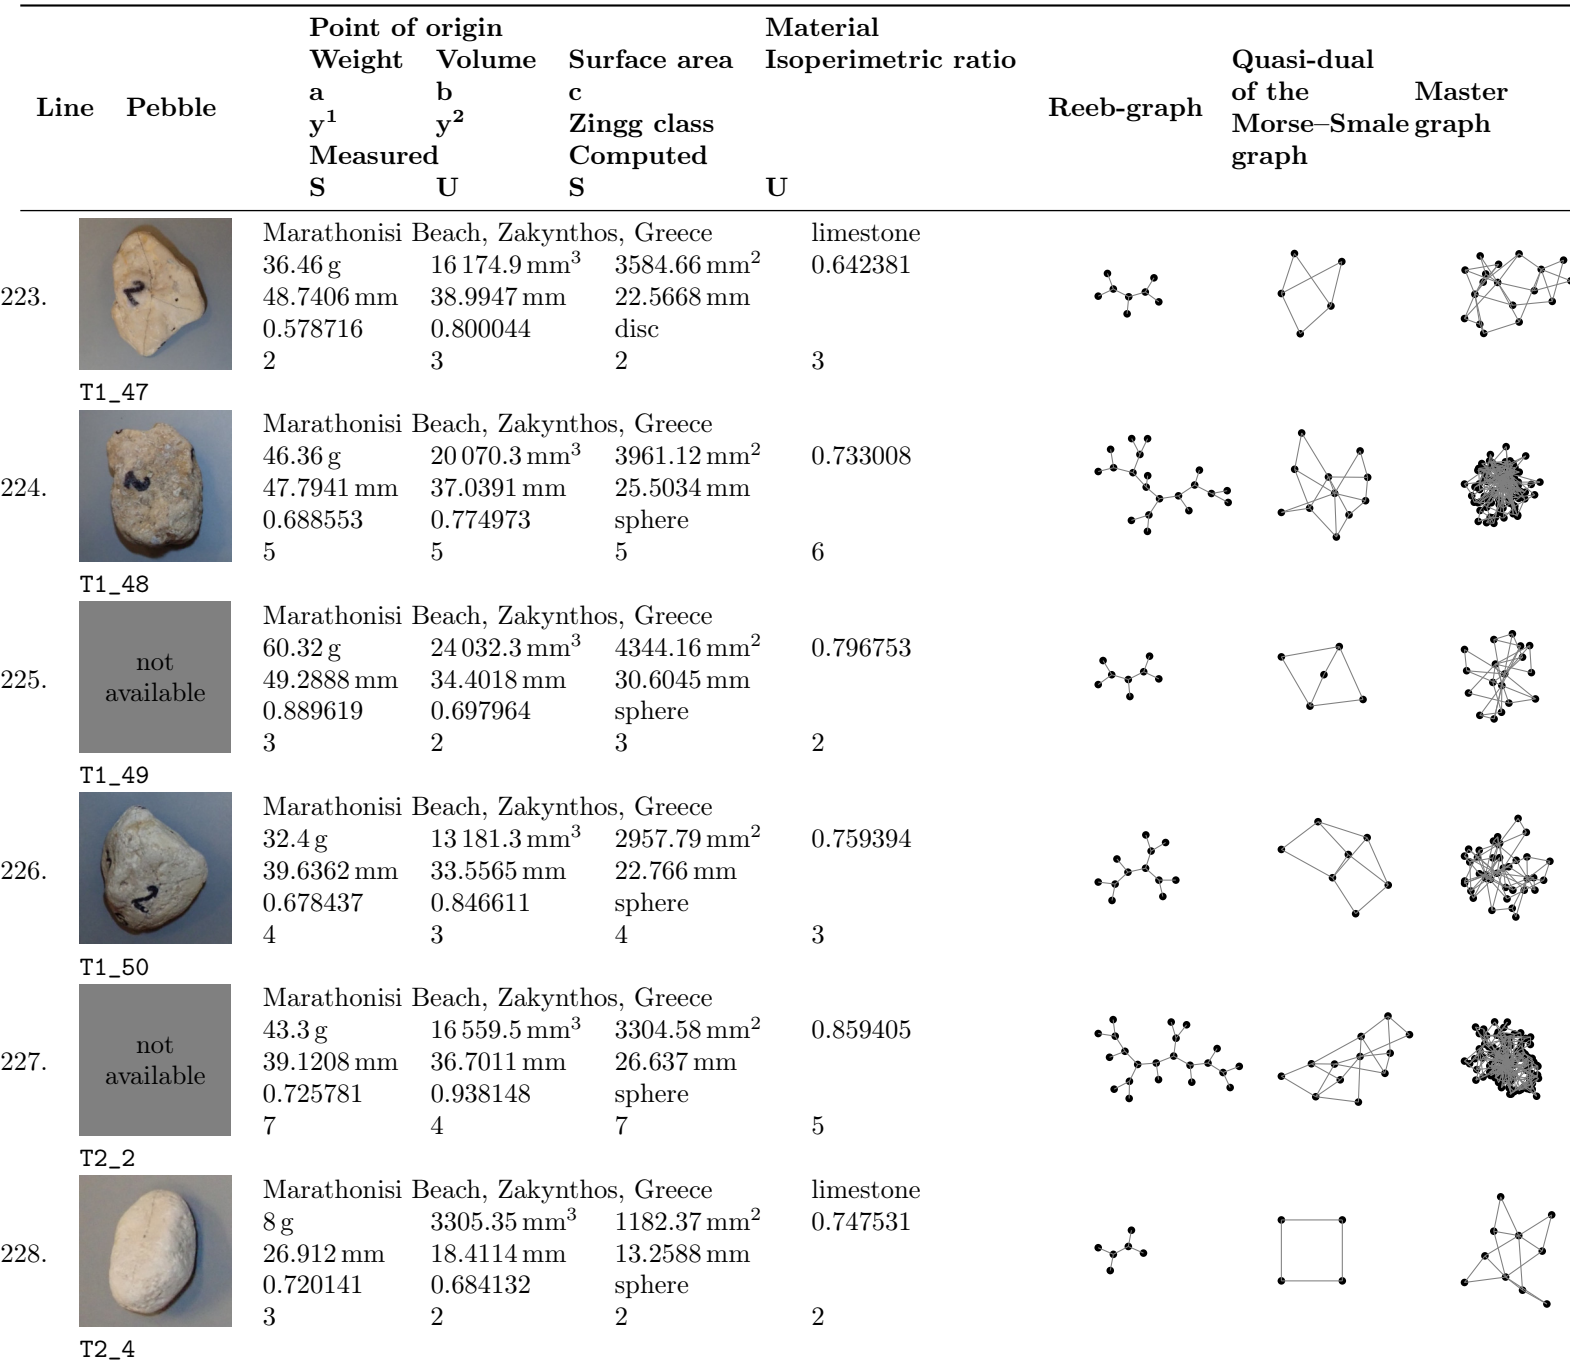  | 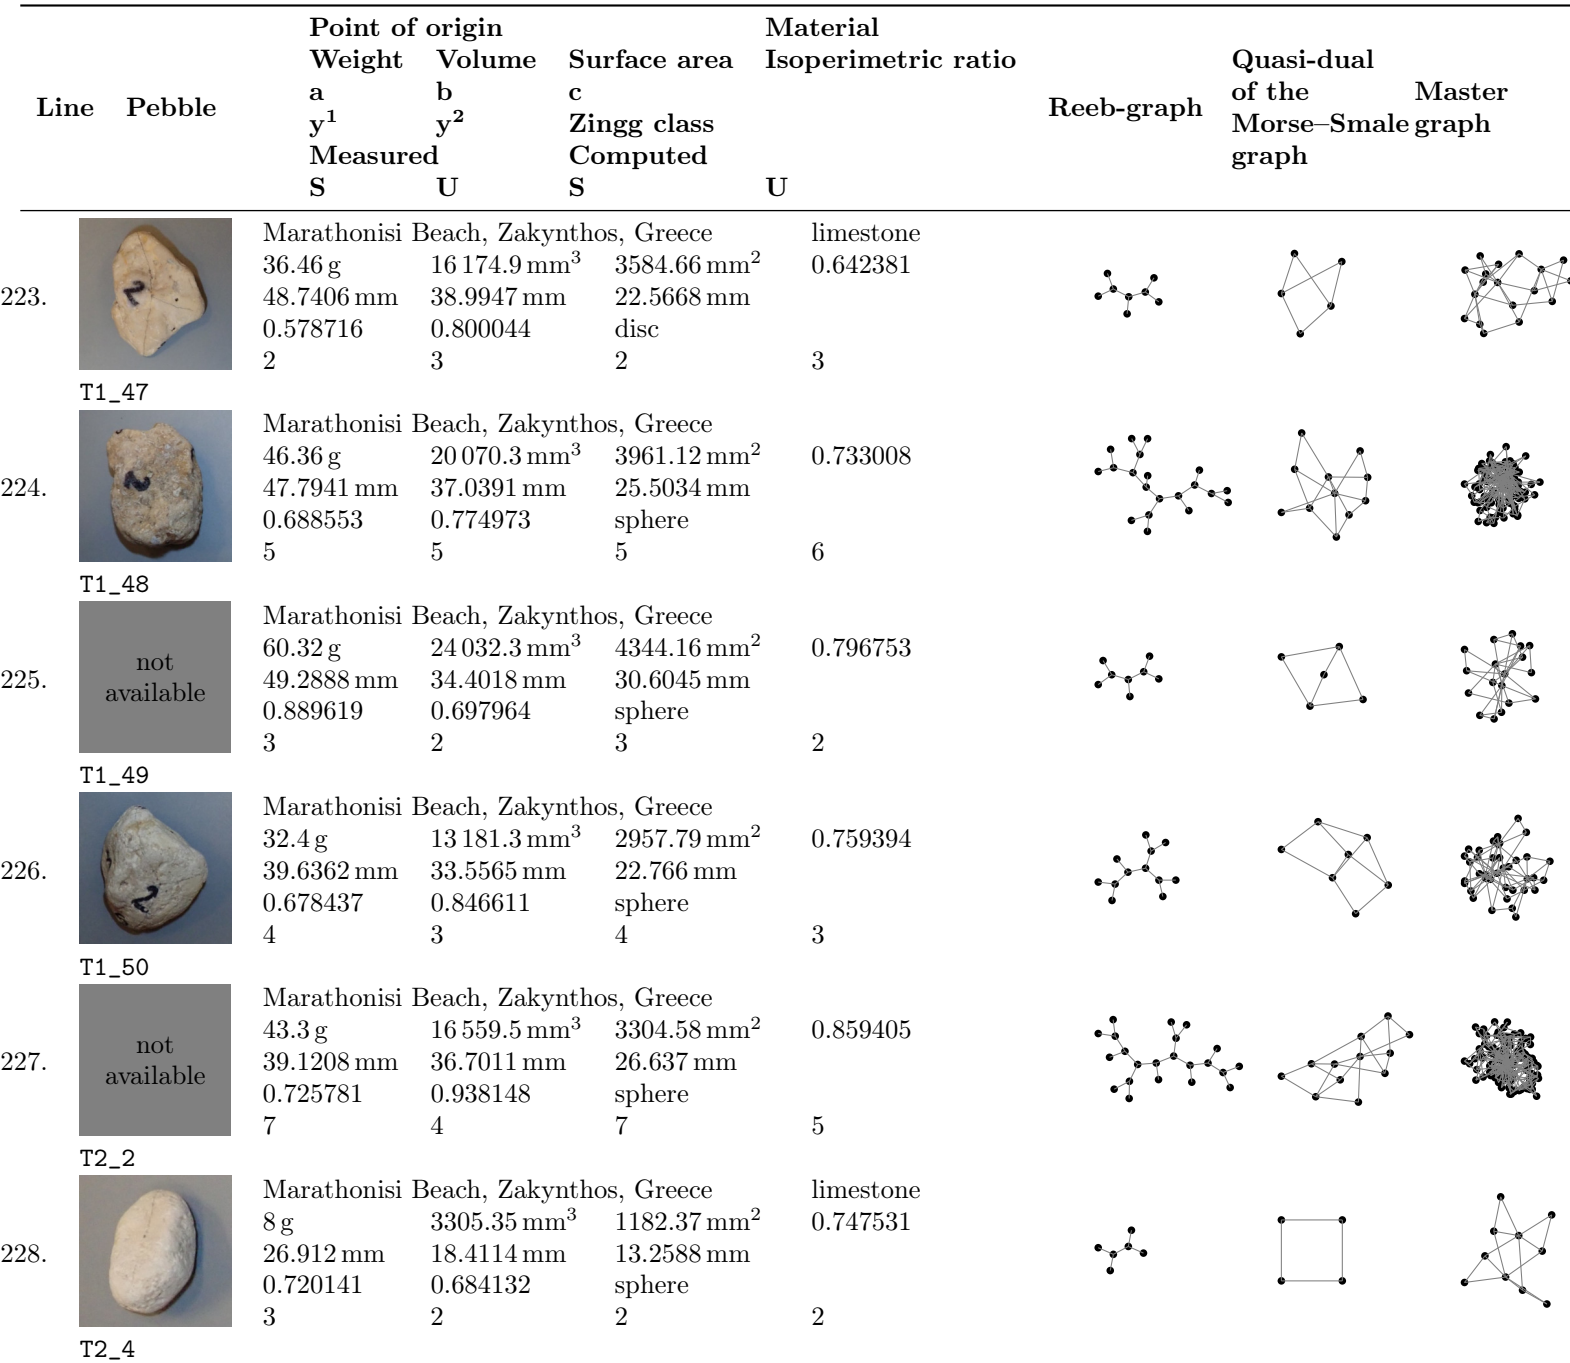  |
|      | T1_50                                                                               |                                                                                |                                                                    |                                                      |                                      |                                                                                       |                                                                                       |                                                                                       |
| 227. | 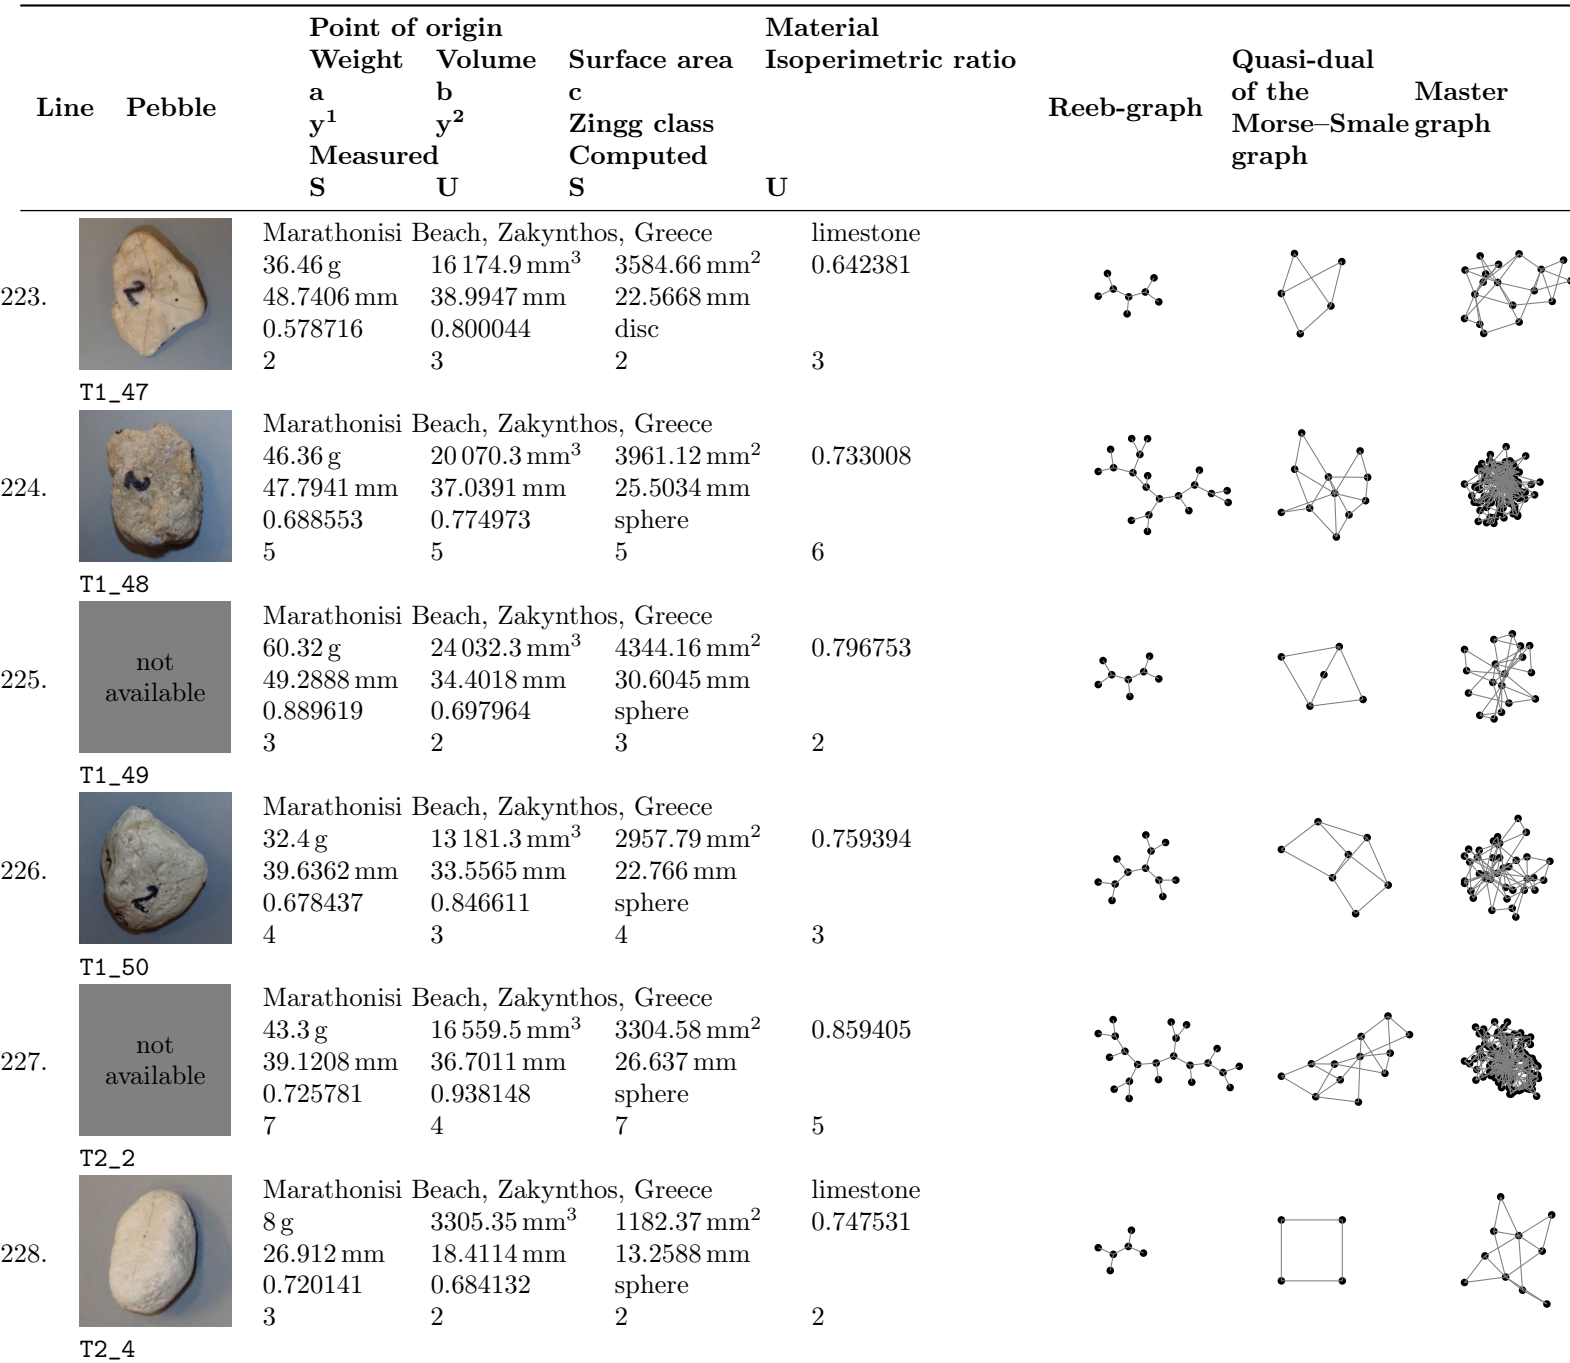 | Marathonisi Beach, Zakynthos, Greece<br>43.3 g<br>39.1208 mm<br>0.725781<br>7  | 43.3 g<br>16 559.5 mm <sup>3</sup><br>36.7011 mm<br>0.938148<br>4  | 3304.58 mm <sup>2</sup><br>26.637 mm<br>sphere<br>7  | 0.859405<br>5                        | 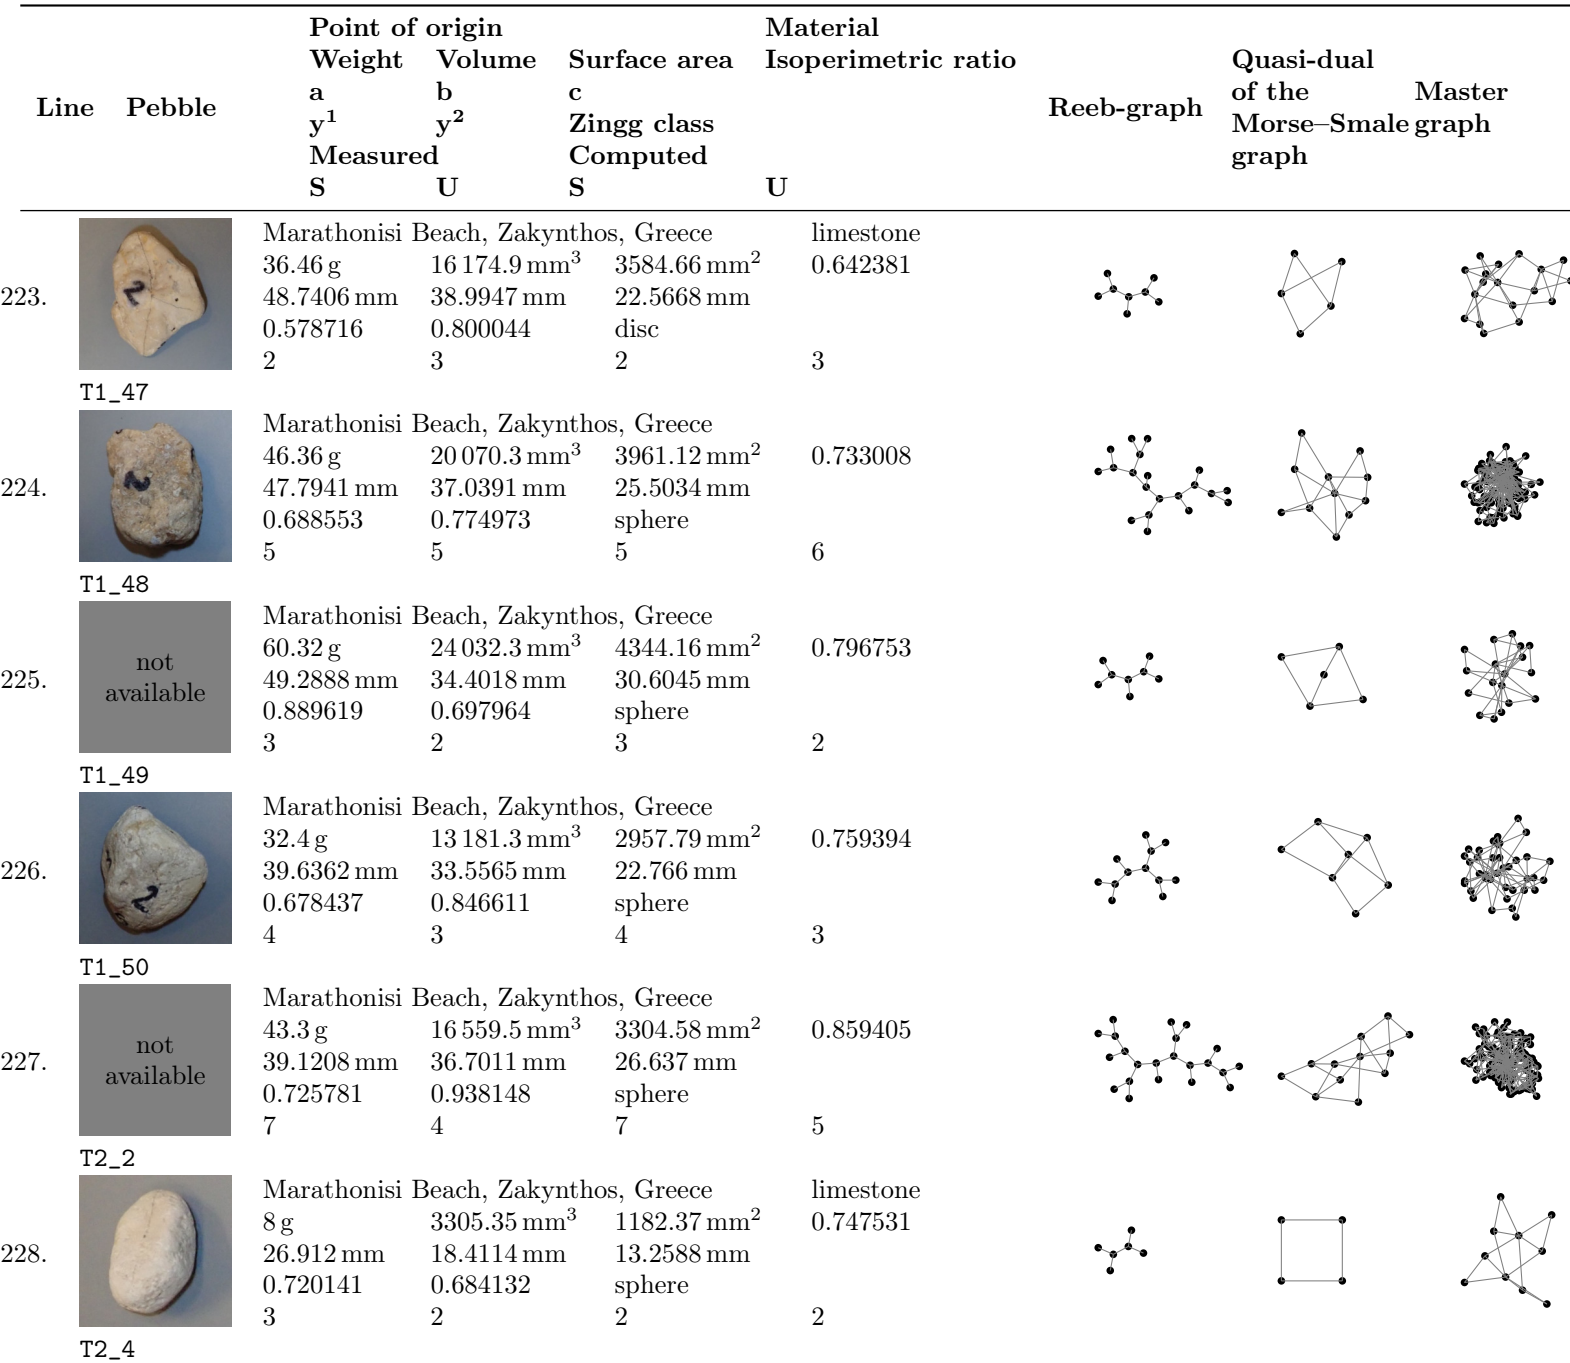 | 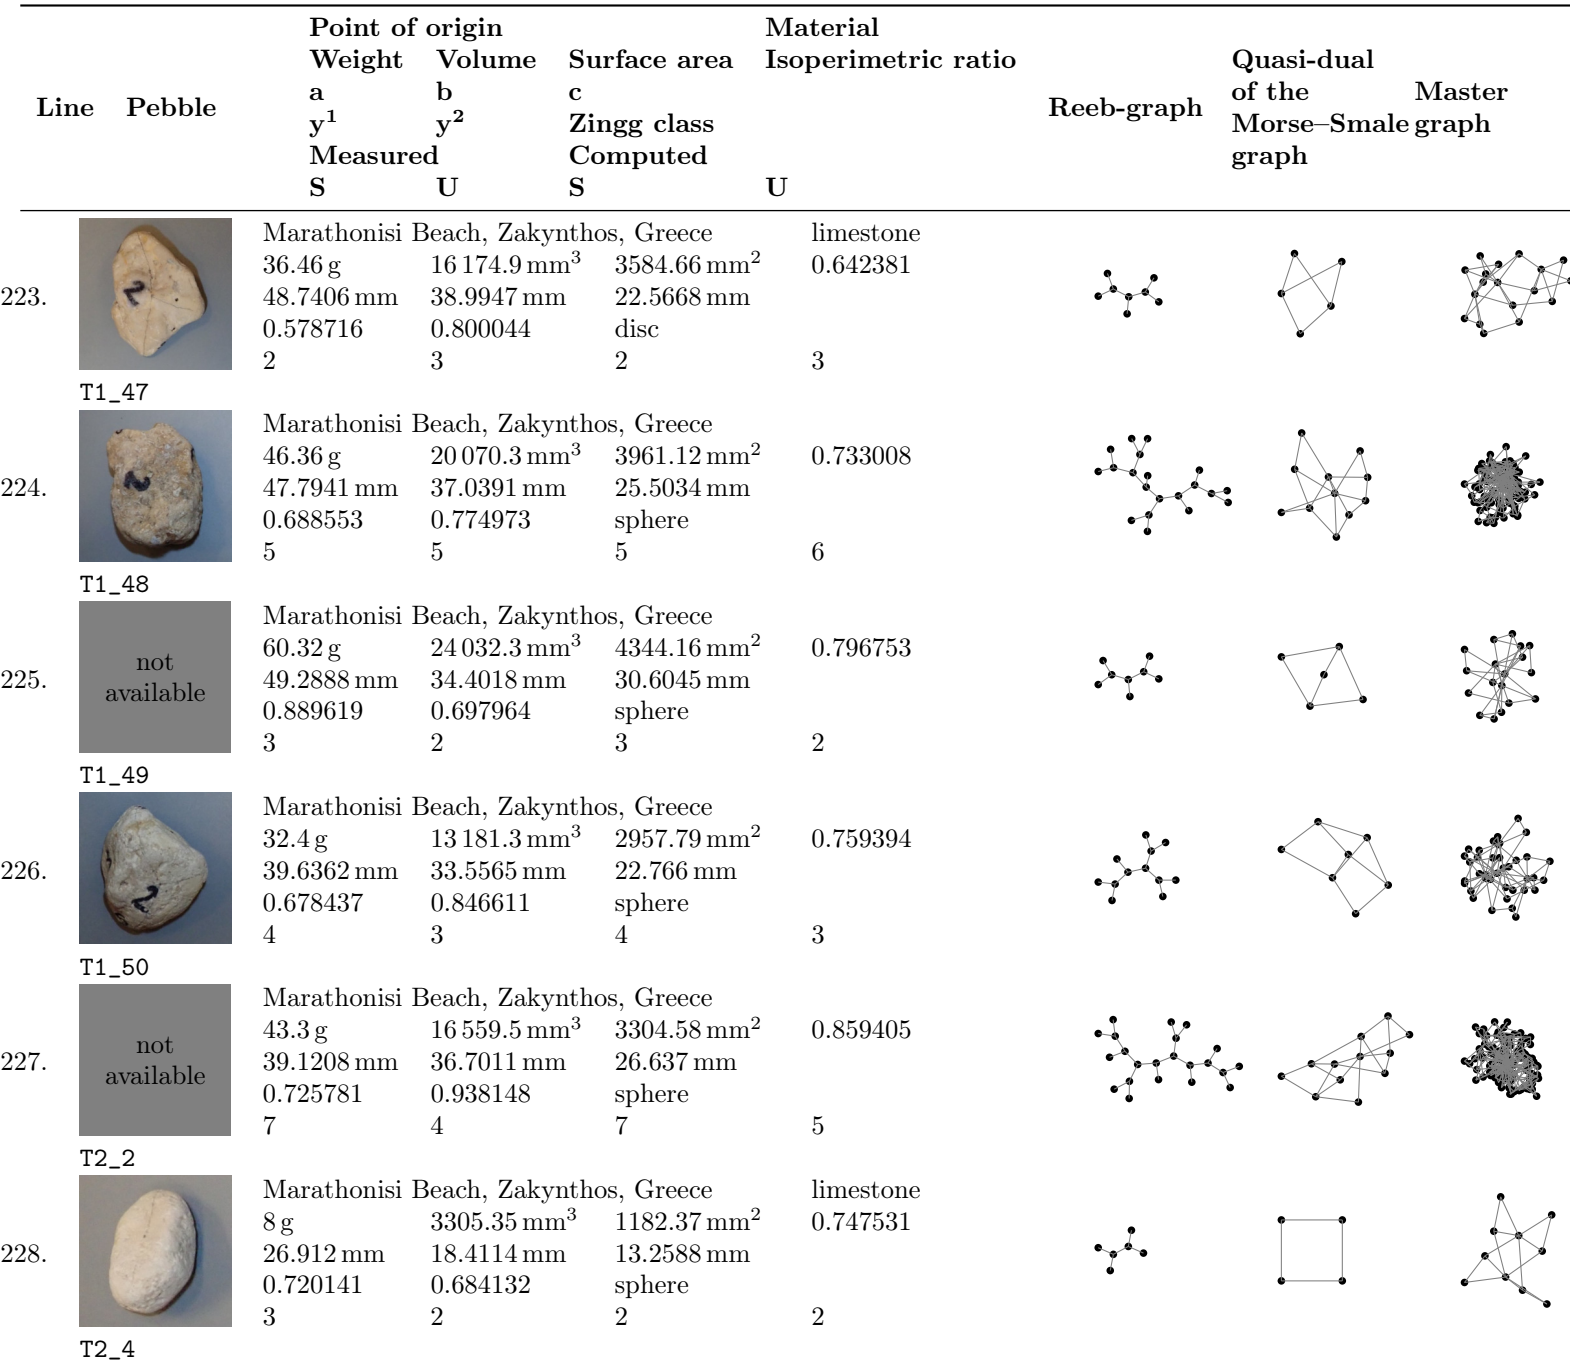 | 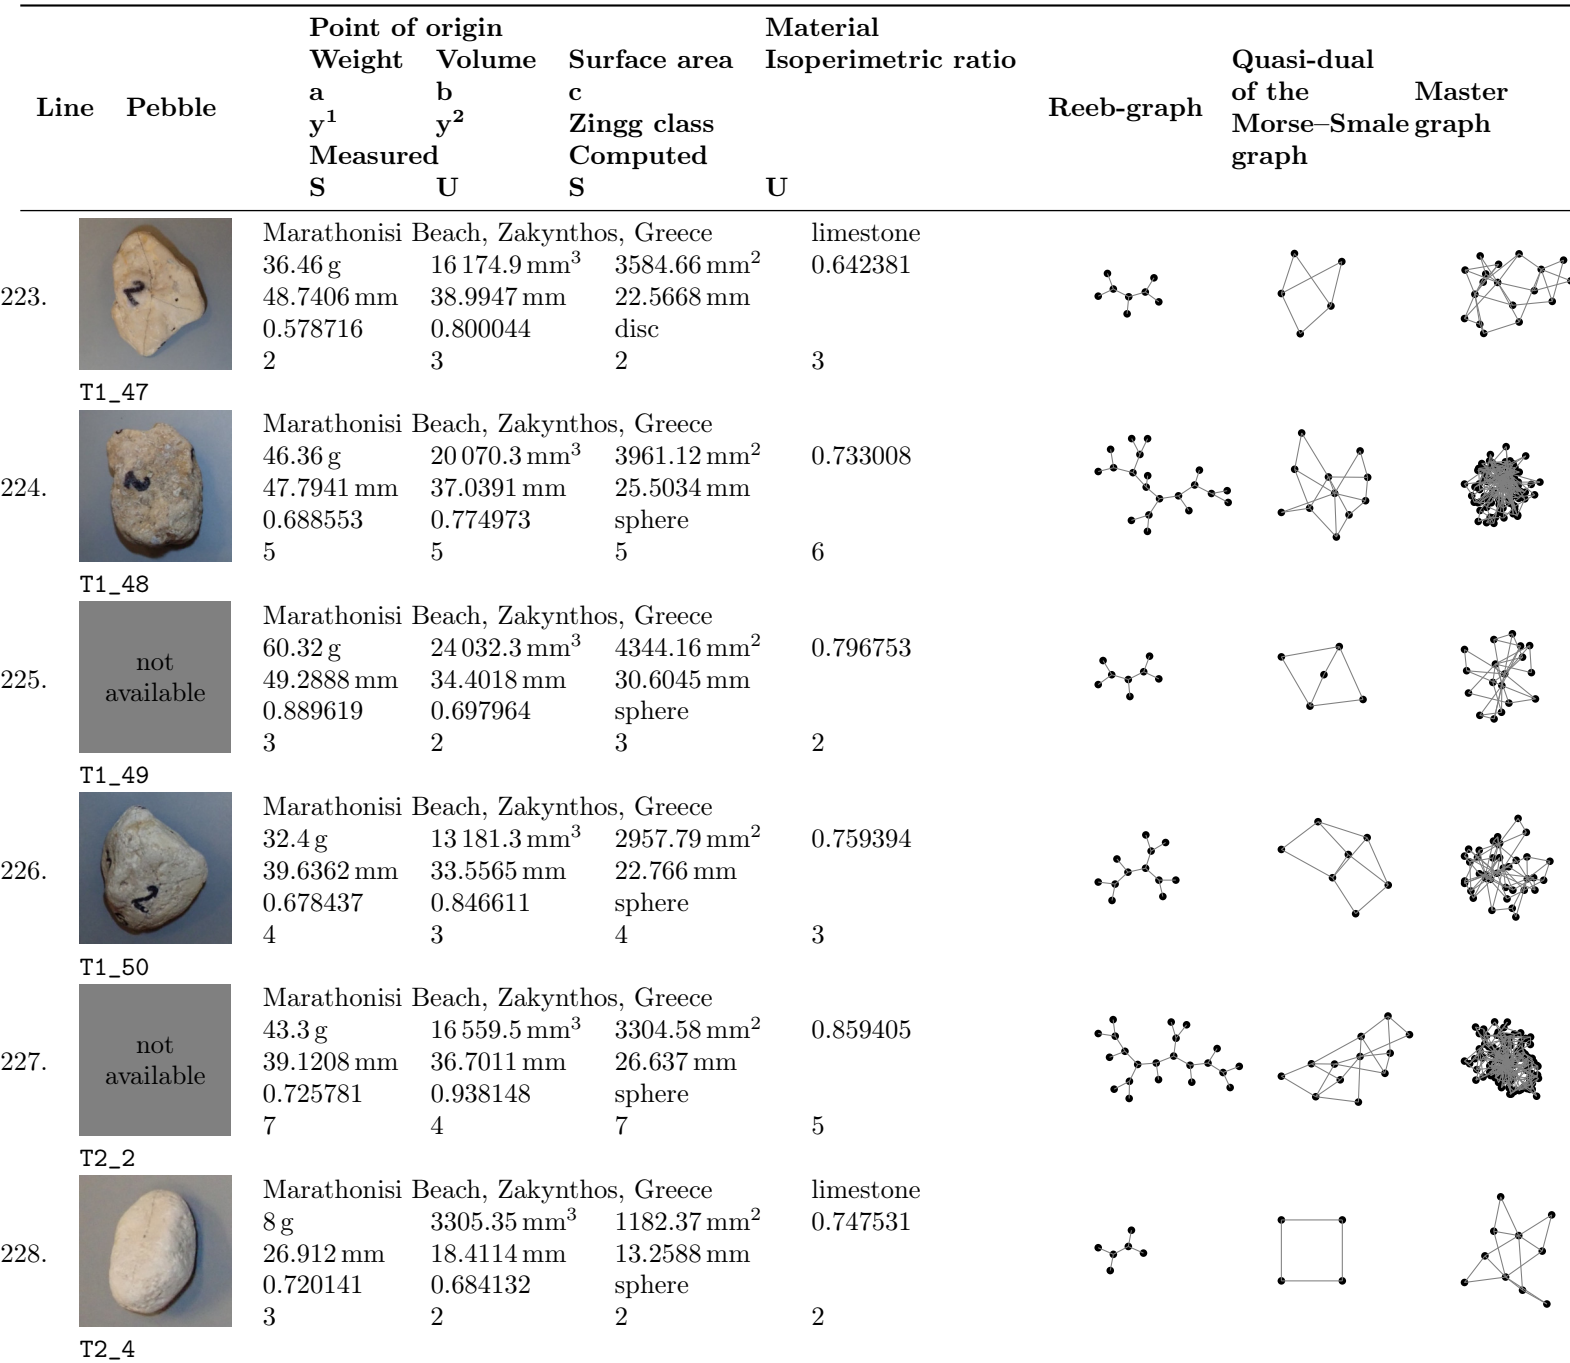 |
|      | T2_2                                                                                |                                                                                |                                                                    |                                                      |                                      |                                                                                       |                                                                                       |                                                                                       |
| 228. | 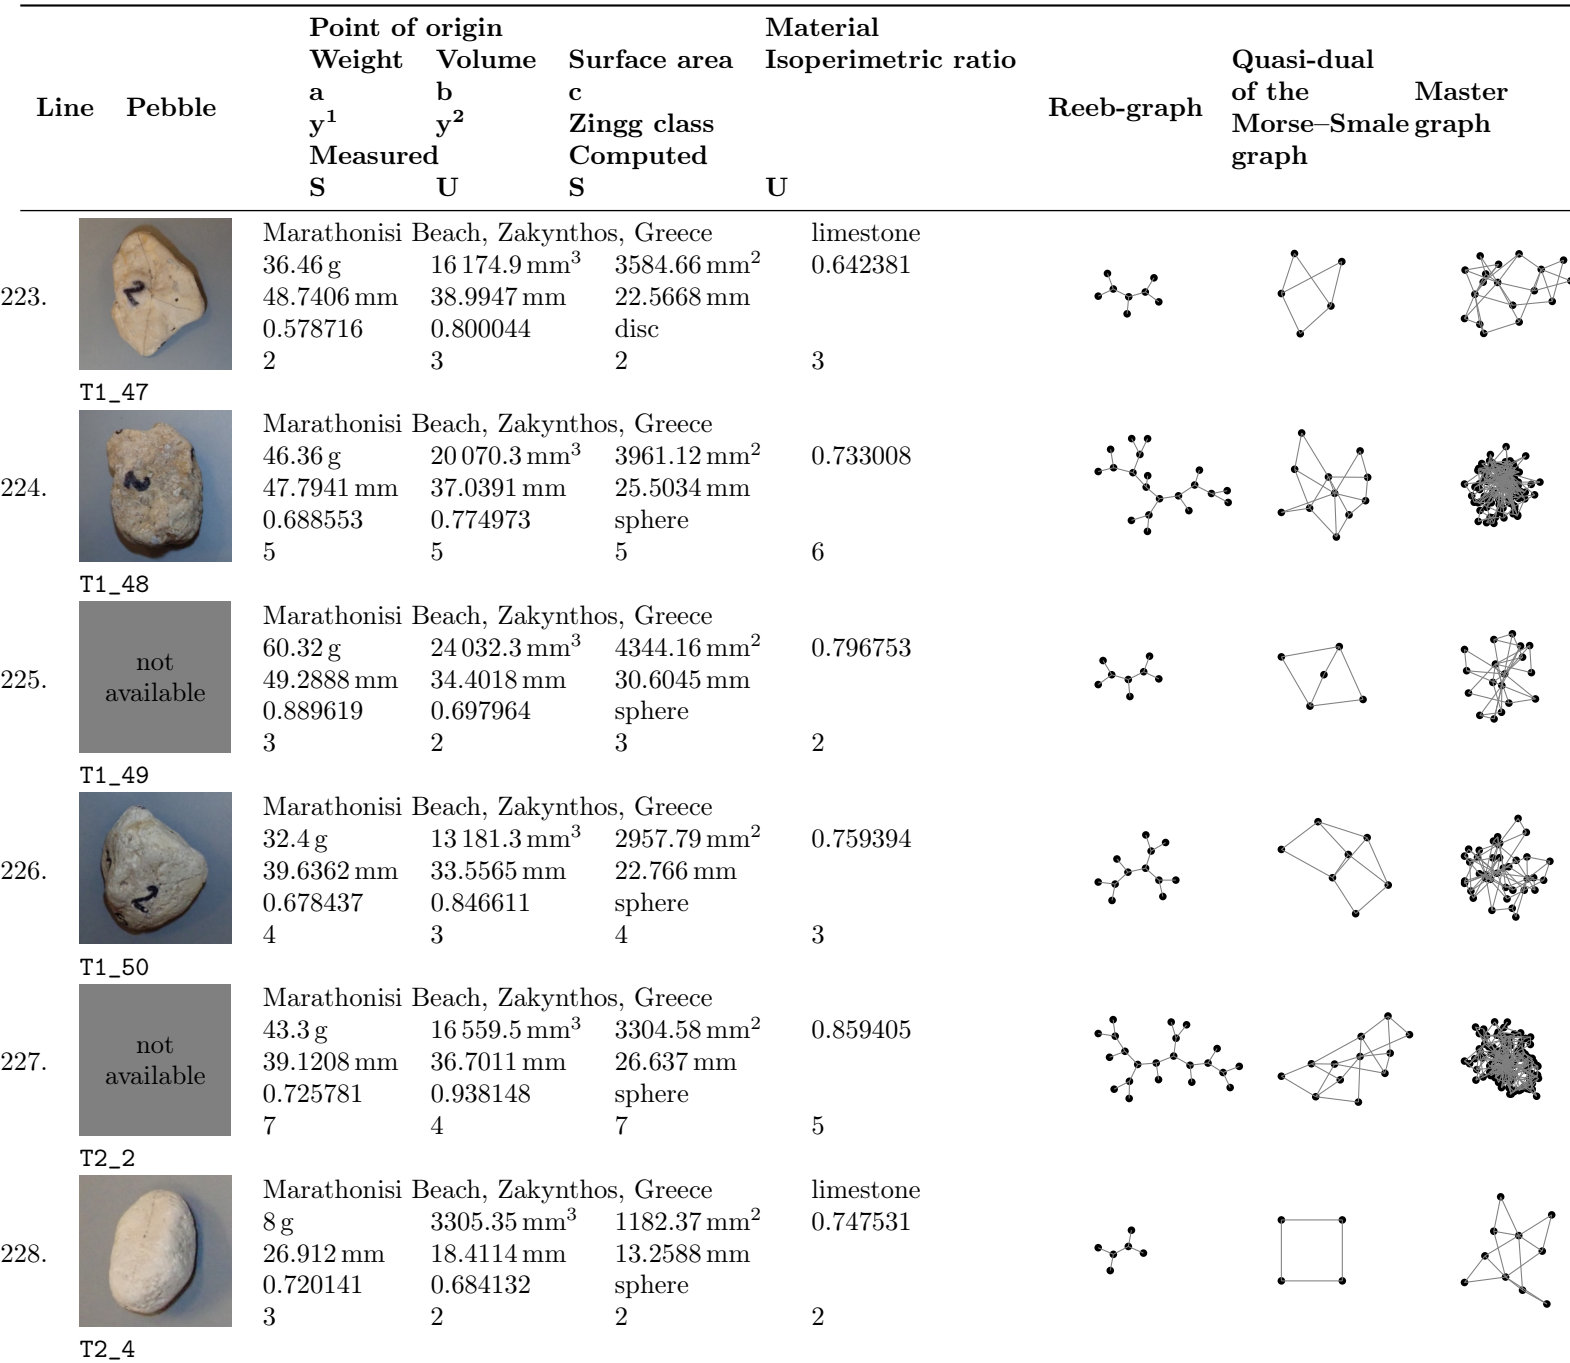 | Marathonisi Beach, Zakynthos, Greece<br>8 g<br>26.912 mm<br>0.720141<br>3      | 8 g<br>3305.35 mm <sup>3</sup><br>18.4114 mm<br>0.684132<br>2      | 1182.37 mm <sup>2</sup><br>13.2588 mm<br>sphere<br>2 | limestone<br>0.747531<br>2           | 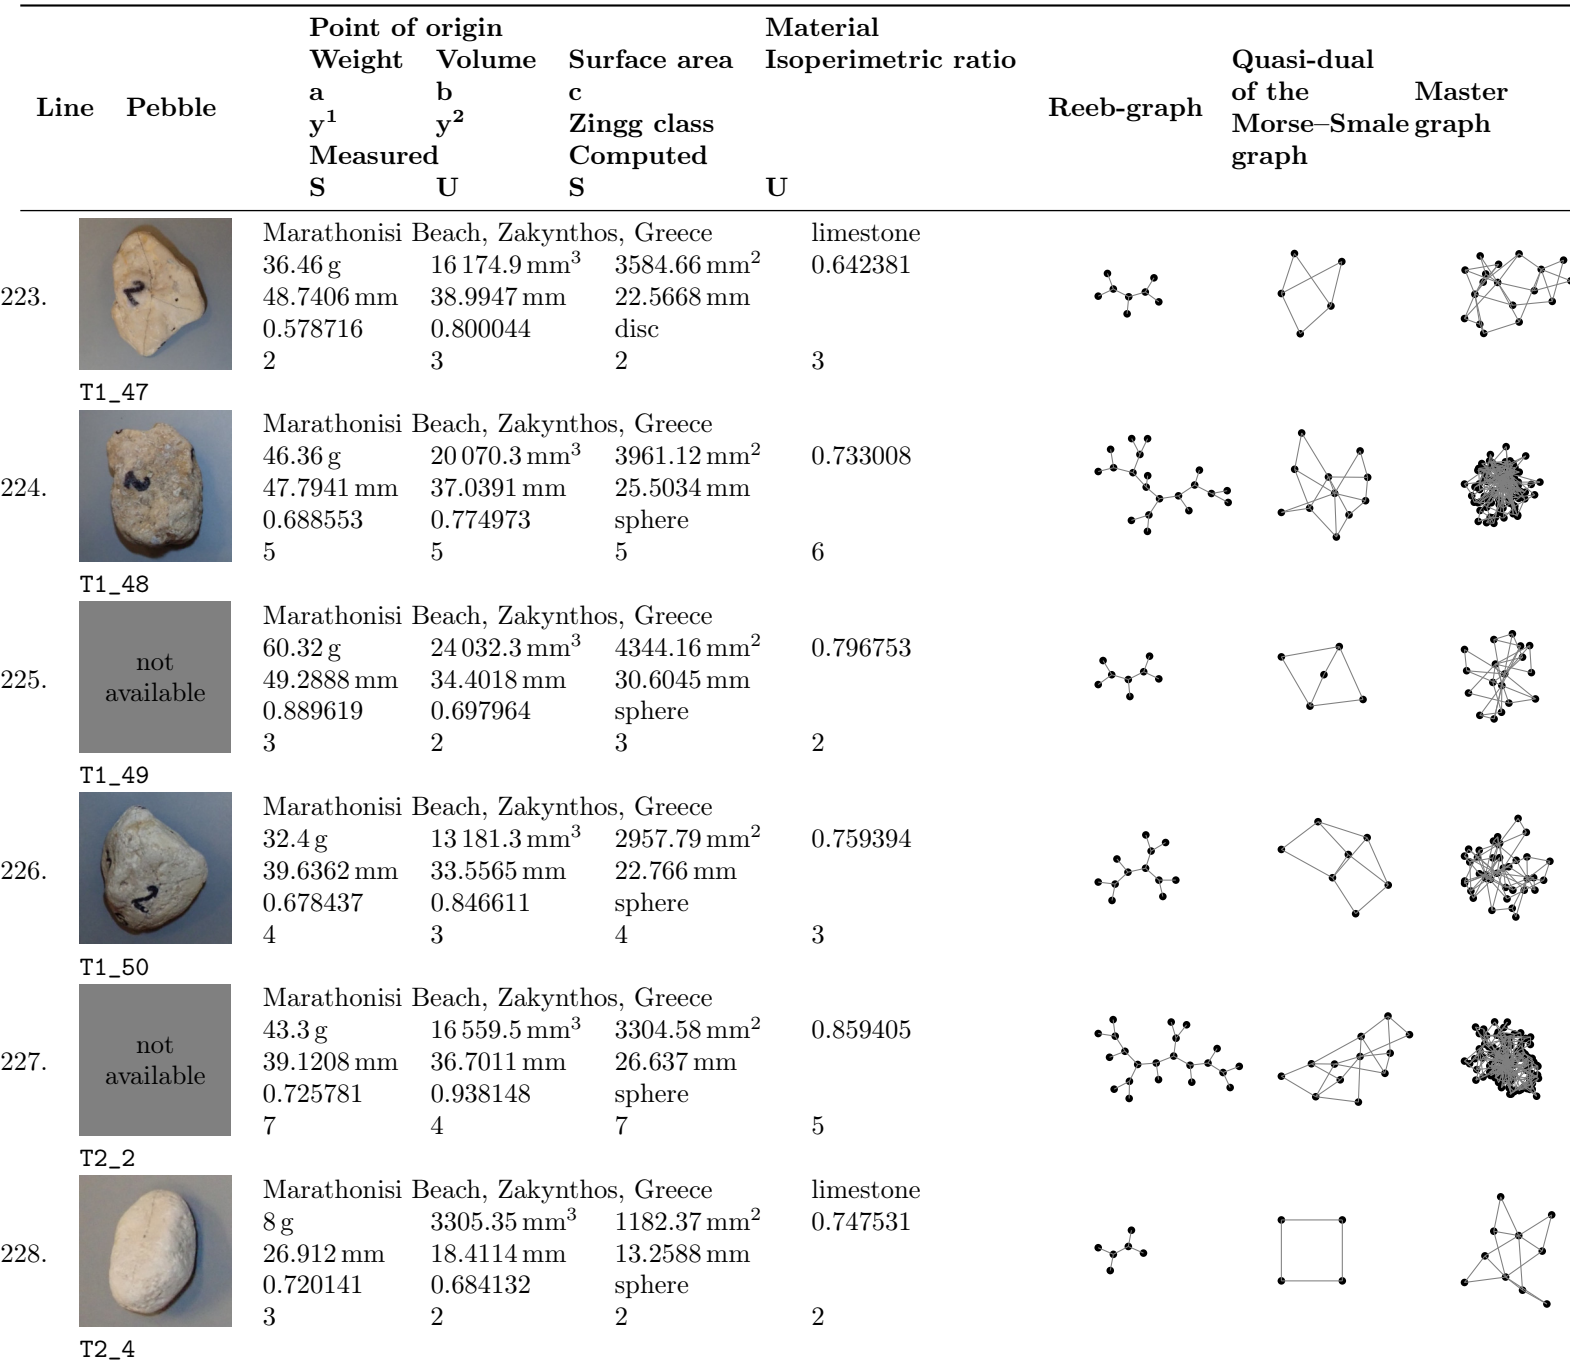 | 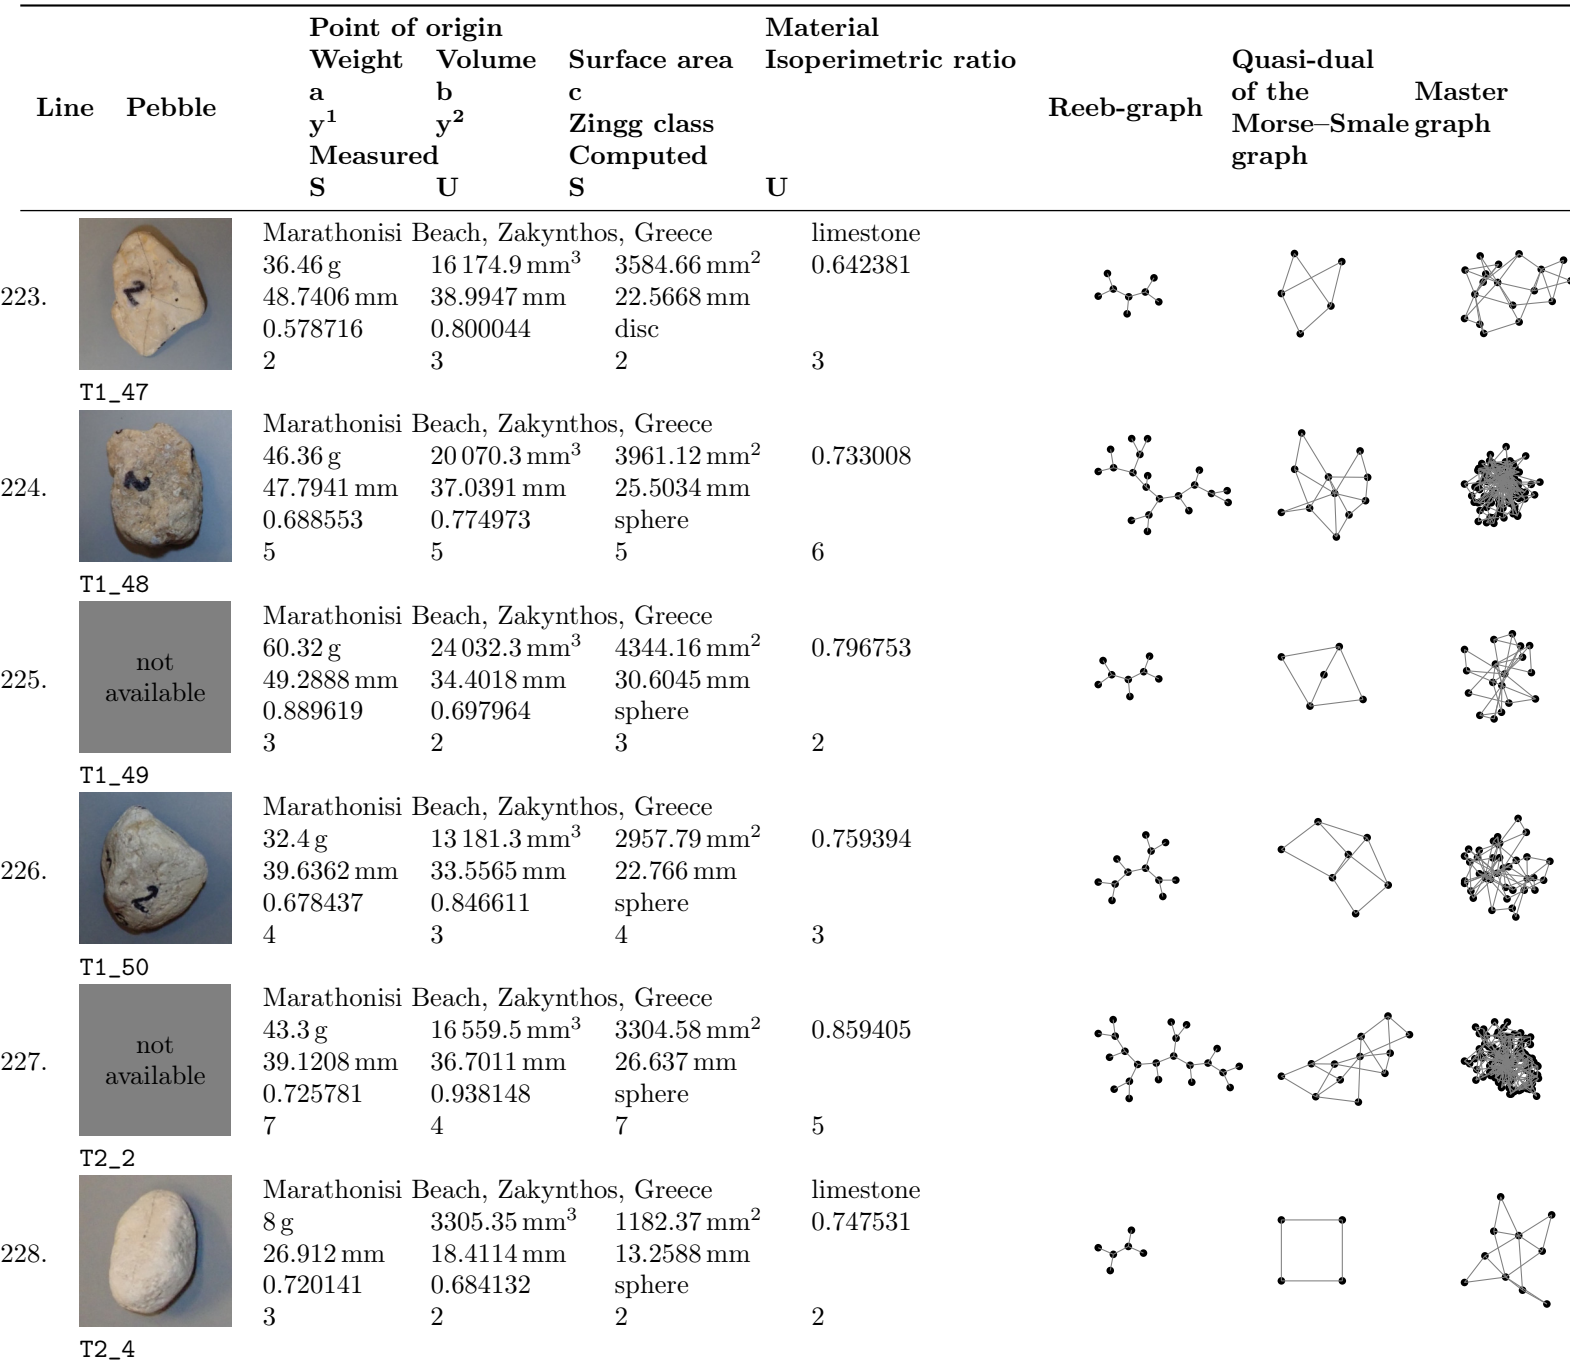 | 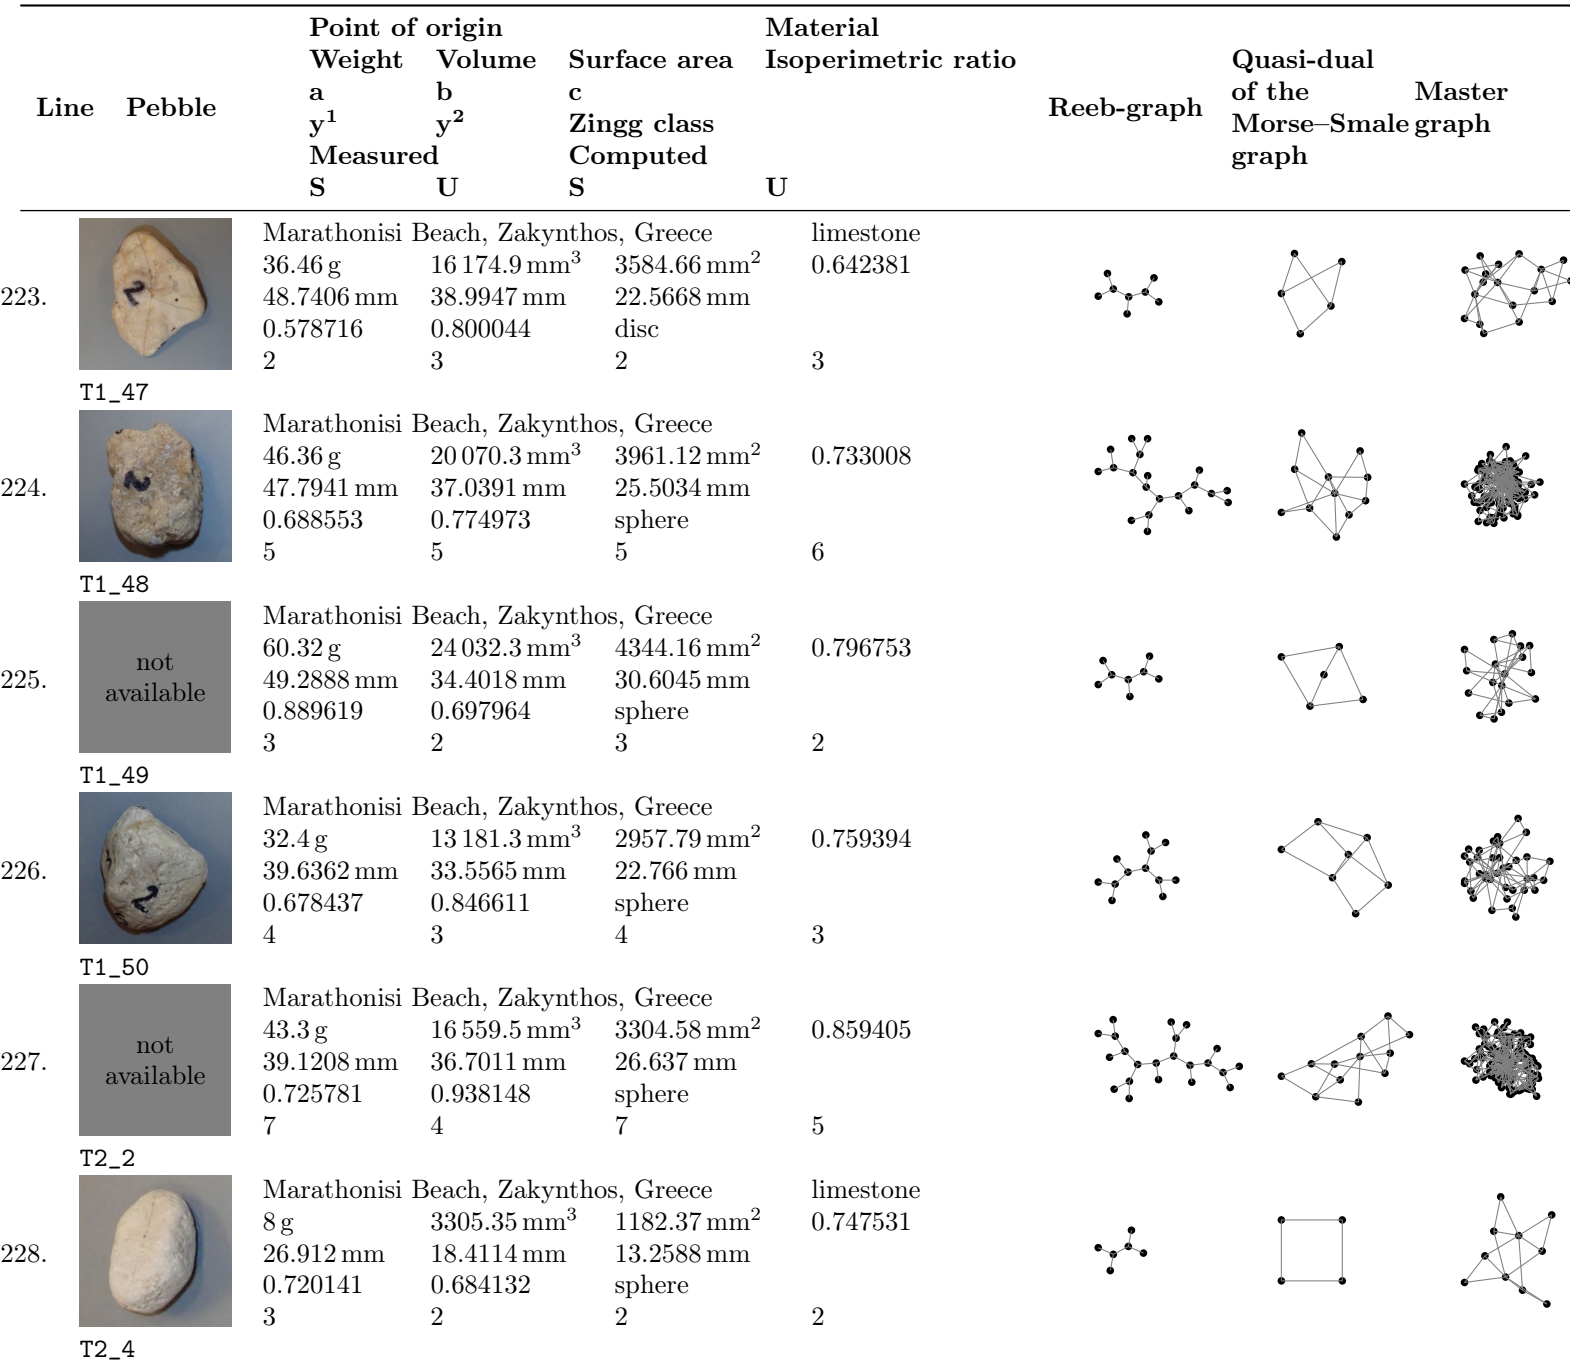 |
|      | T2_4                                                                                |                                                                                |                                                                    |                                                      |                                      |                                                                                       |                                                                                       |                                                                                       |

| Line | Pebble                                                                              | Point of origin                      |                         |                              | Material              | Reeb-graph                                                                            | Quasi-dual<br>of the<br>Morse–Smale<br>graph                                          | Master<br>graph                                                                       |
|------|-------------------------------------------------------------------------------------|--------------------------------------|-------------------------|------------------------------|-----------------------|---------------------------------------------------------------------------------------|---------------------------------------------------------------------------------------|---------------------------------------------------------------------------------------|
|      |                                                                                     | Weight                               | Volume                  | Surface area                 |                       |                                                                                       |                                                                                       |                                                                                       |
|      |                                                                                     | a                                    | b                       | c                            |                       |                                                                                       |                                                                                       |                                                                                       |
|      |                                                                                     | y <sup>1</sup><br>Measured<br>S      | y <sup>2</sup><br>U     | Zingg class<br>Computed<br>S |                       |                                                                                       |                                                                                       |                                                                                       |
| 229. | 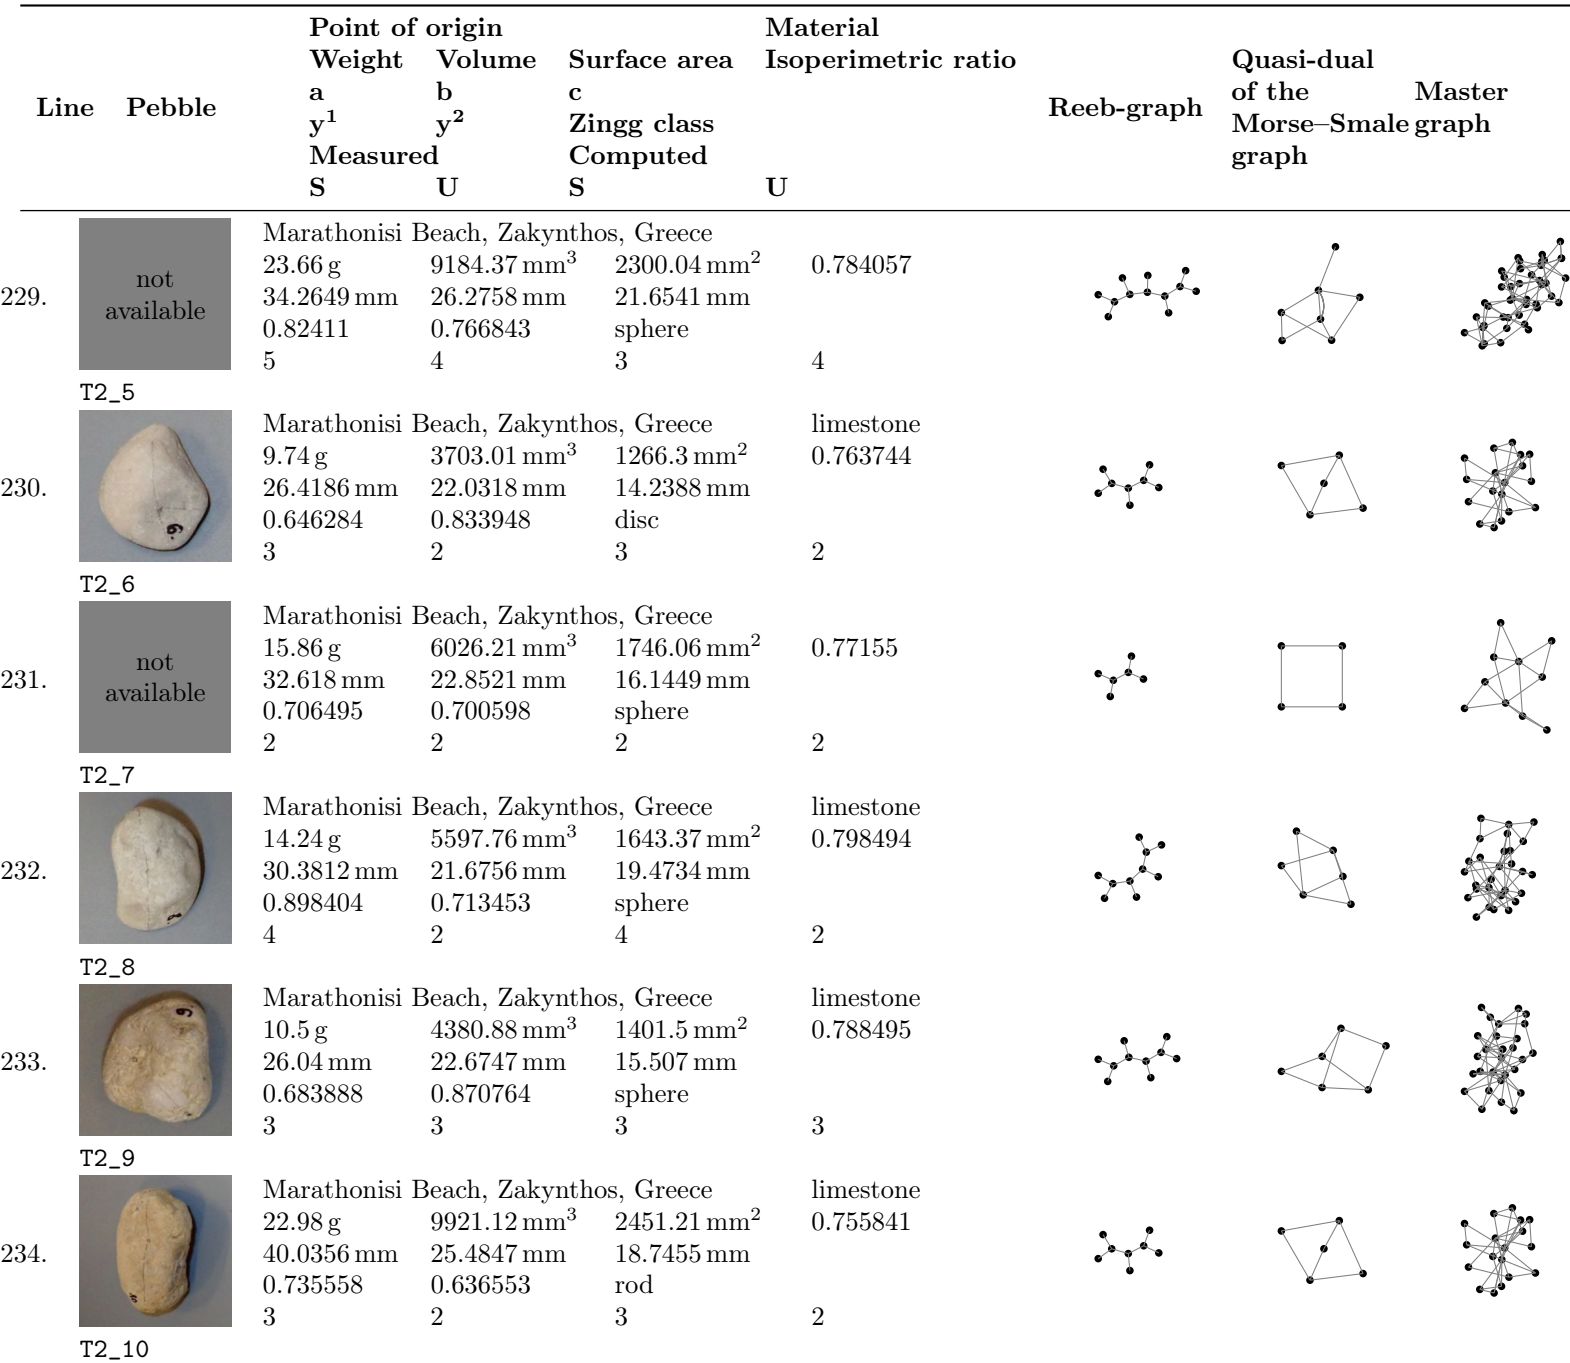   | Marathonisi Beach, Zakynthos, Greece |                         |                              | 0.784057              | 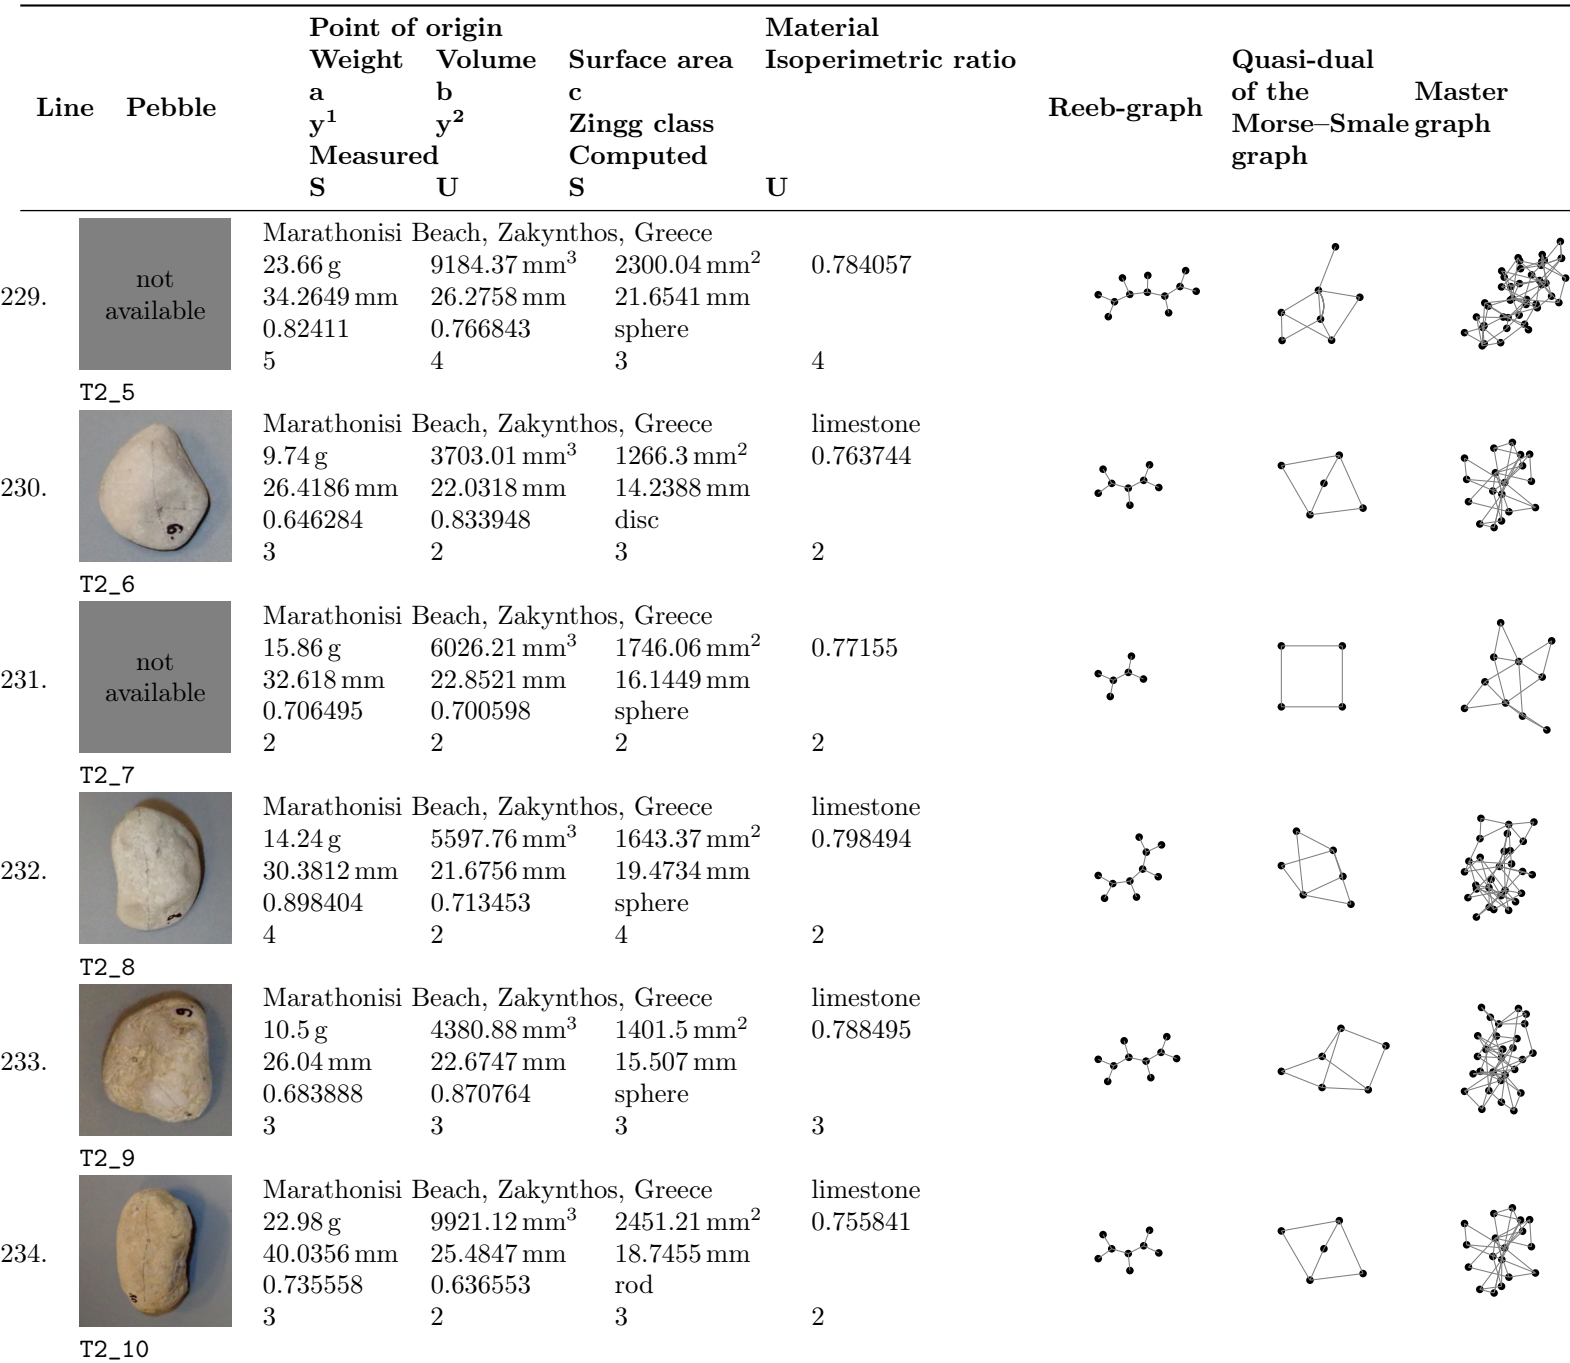   | 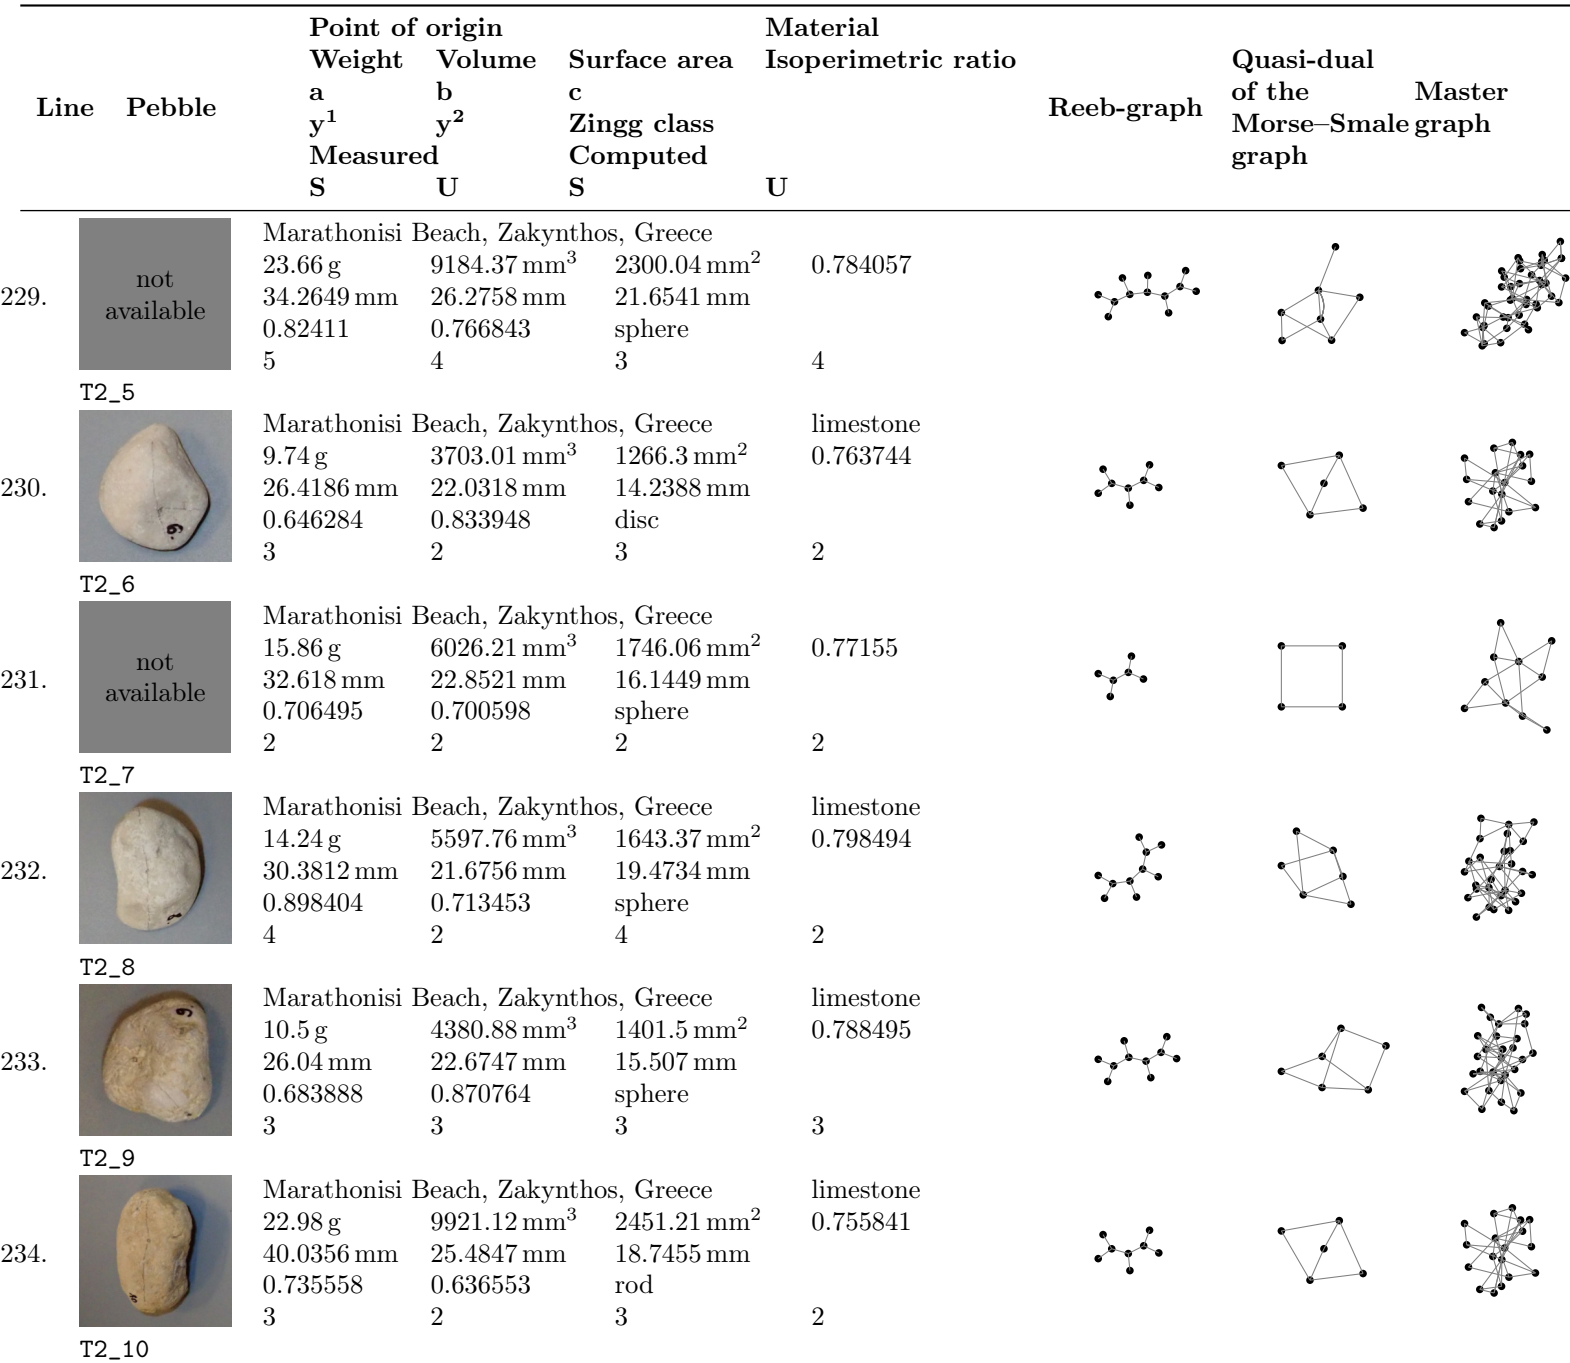   | 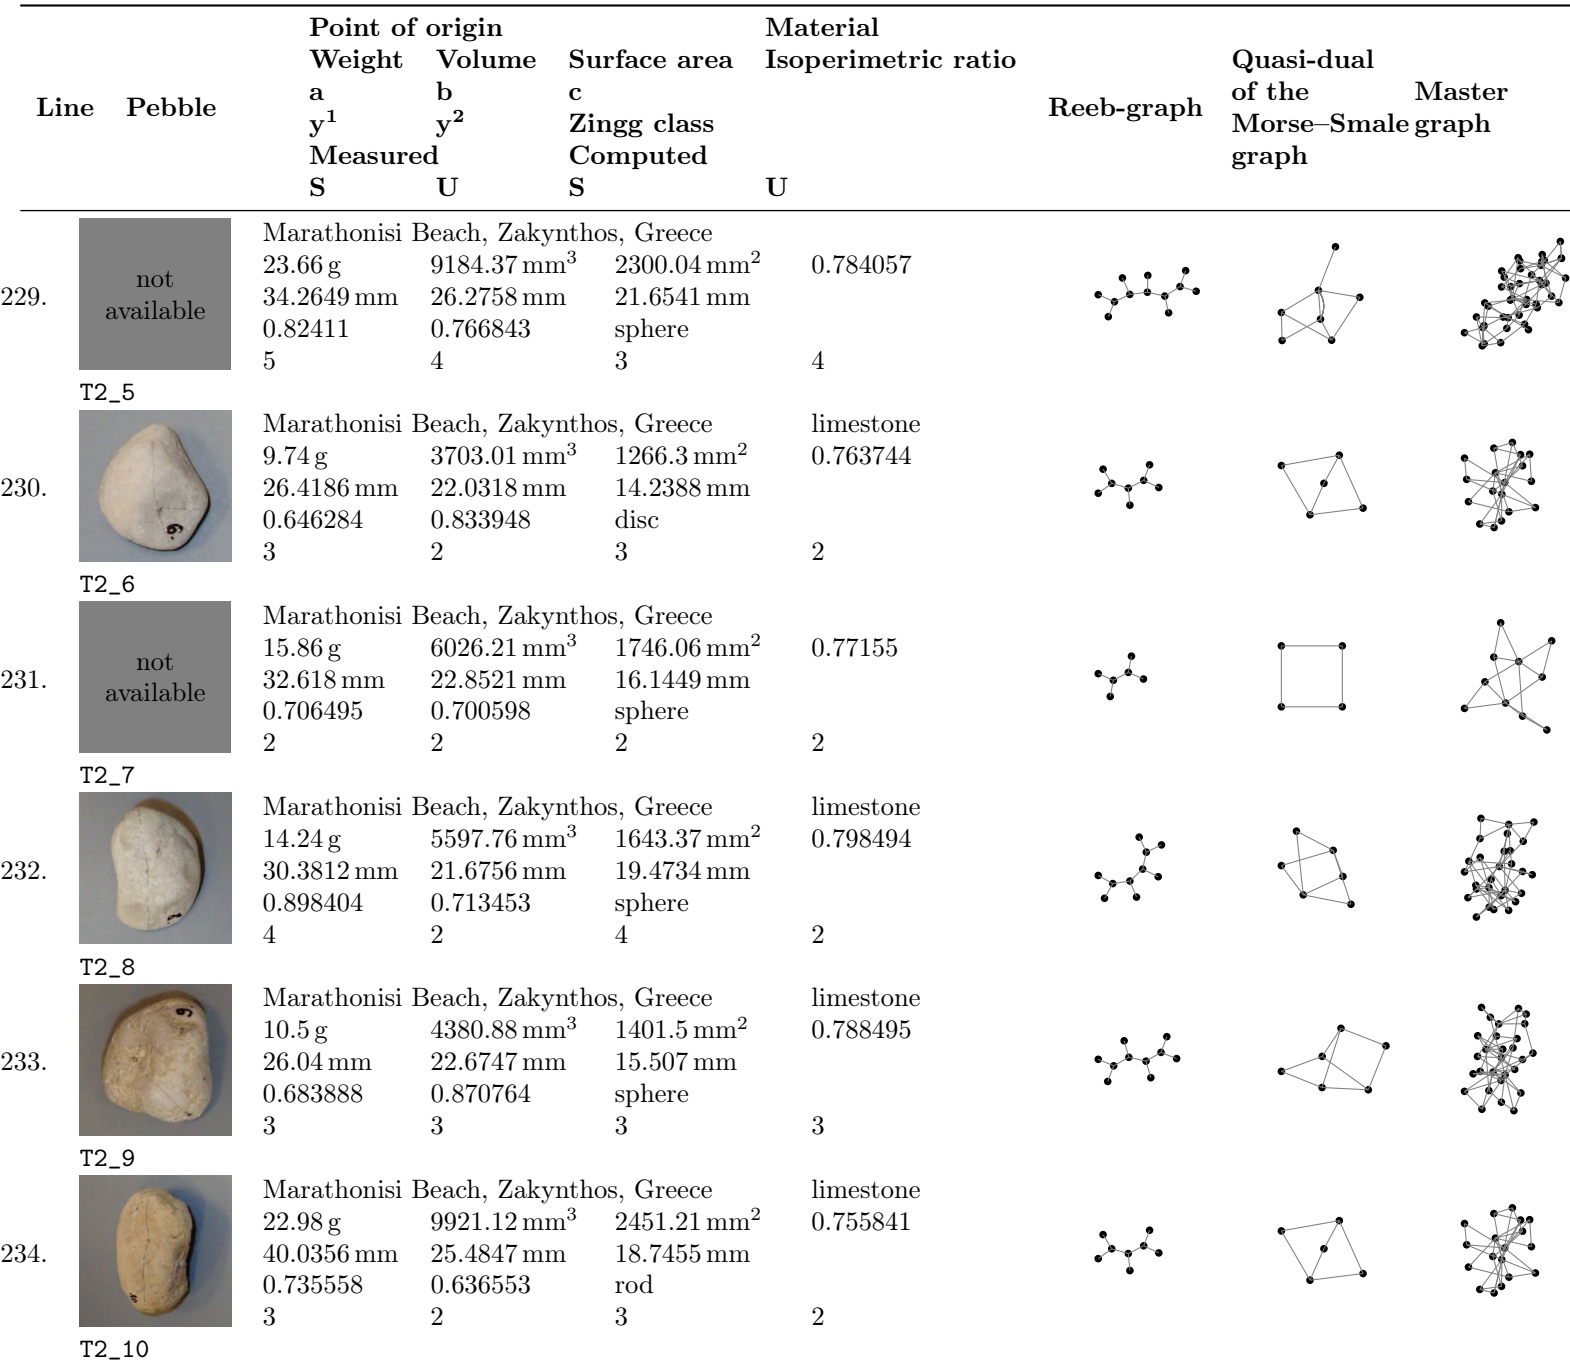   |
|      |                                                                                     | 23.66 g                              | 9184.37 mm <sup>3</sup> | 2300.04 mm <sup>2</sup>      |                       |                                                                                       |                                                                                       |                                                                                       |
|      |                                                                                     | 34.2649 mm                           | 26.2758 mm              | 21.6541 mm                   |                       |                                                                                       |                                                                                       |                                                                                       |
|      |                                                                                     | 0.82411                              | 0.766843                | sphere                       |                       |                                                                                       |                                                                                       |                                                                                       |
|      |                                                                                     | 5                                    | 4                       | 3                            |                       |                                                                                       |                                                                                       |                                                                                       |
|      | T2_5                                                                                |                                      |                         |                              | 4                     |                                                                                       |                                                                                       |                                                                                       |
| 230. | 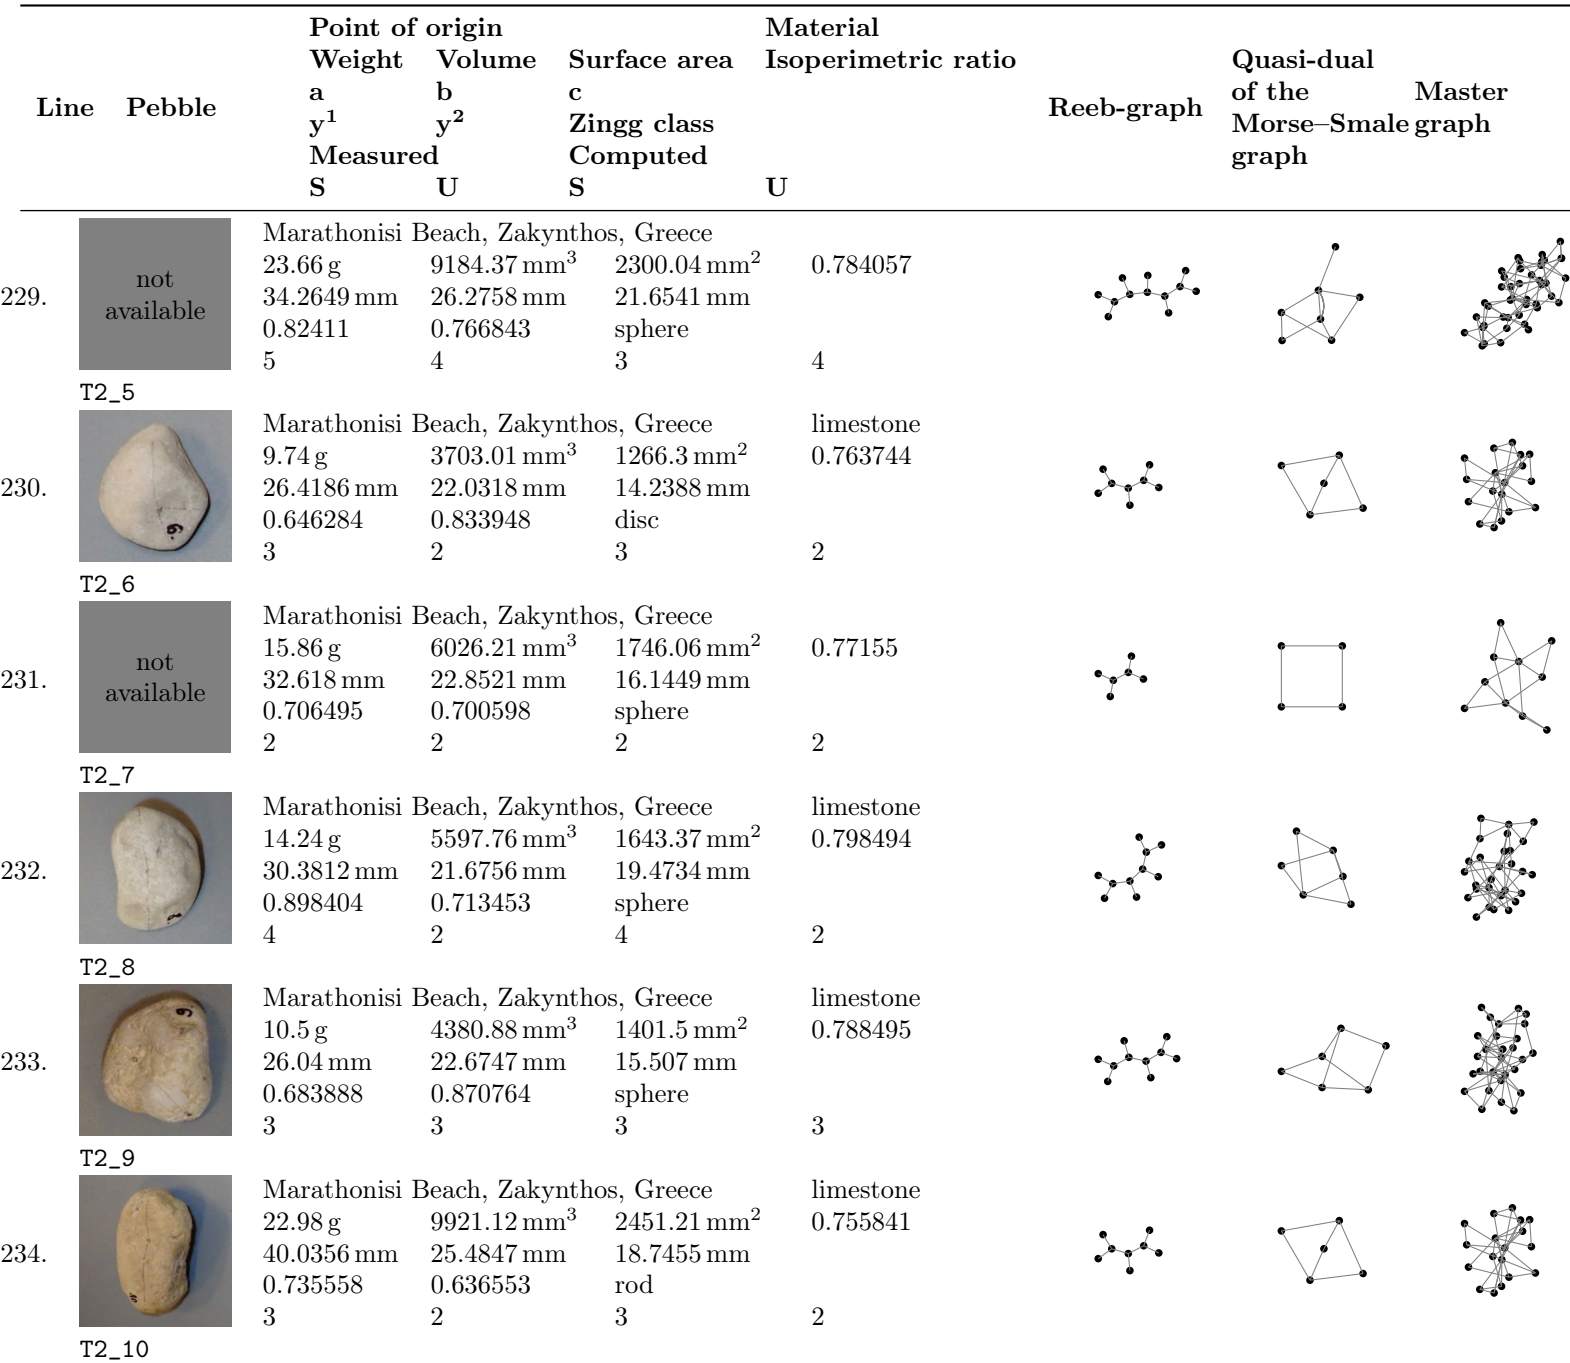   | Marathonisi Beach, Zakynthos, Greece |                         |                              | limestone<br>0.763744 | 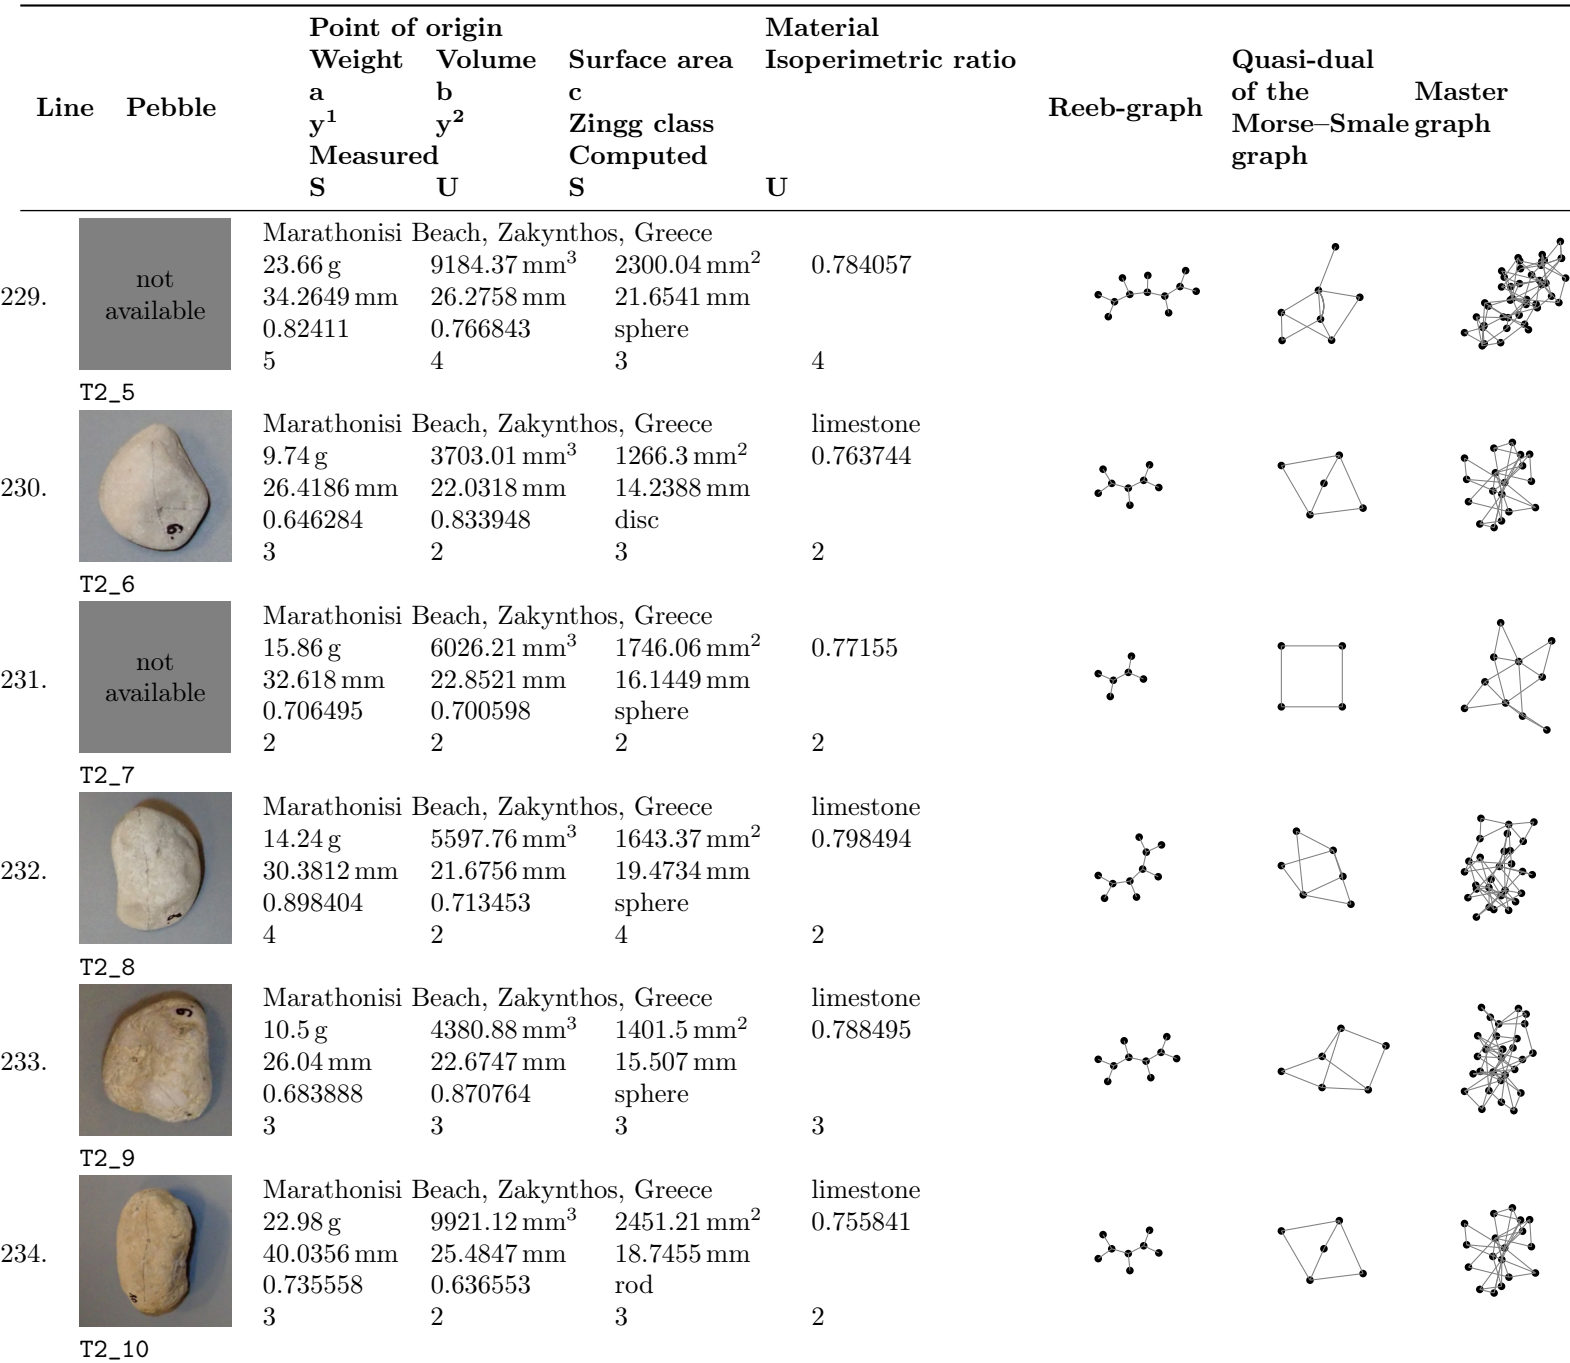   | 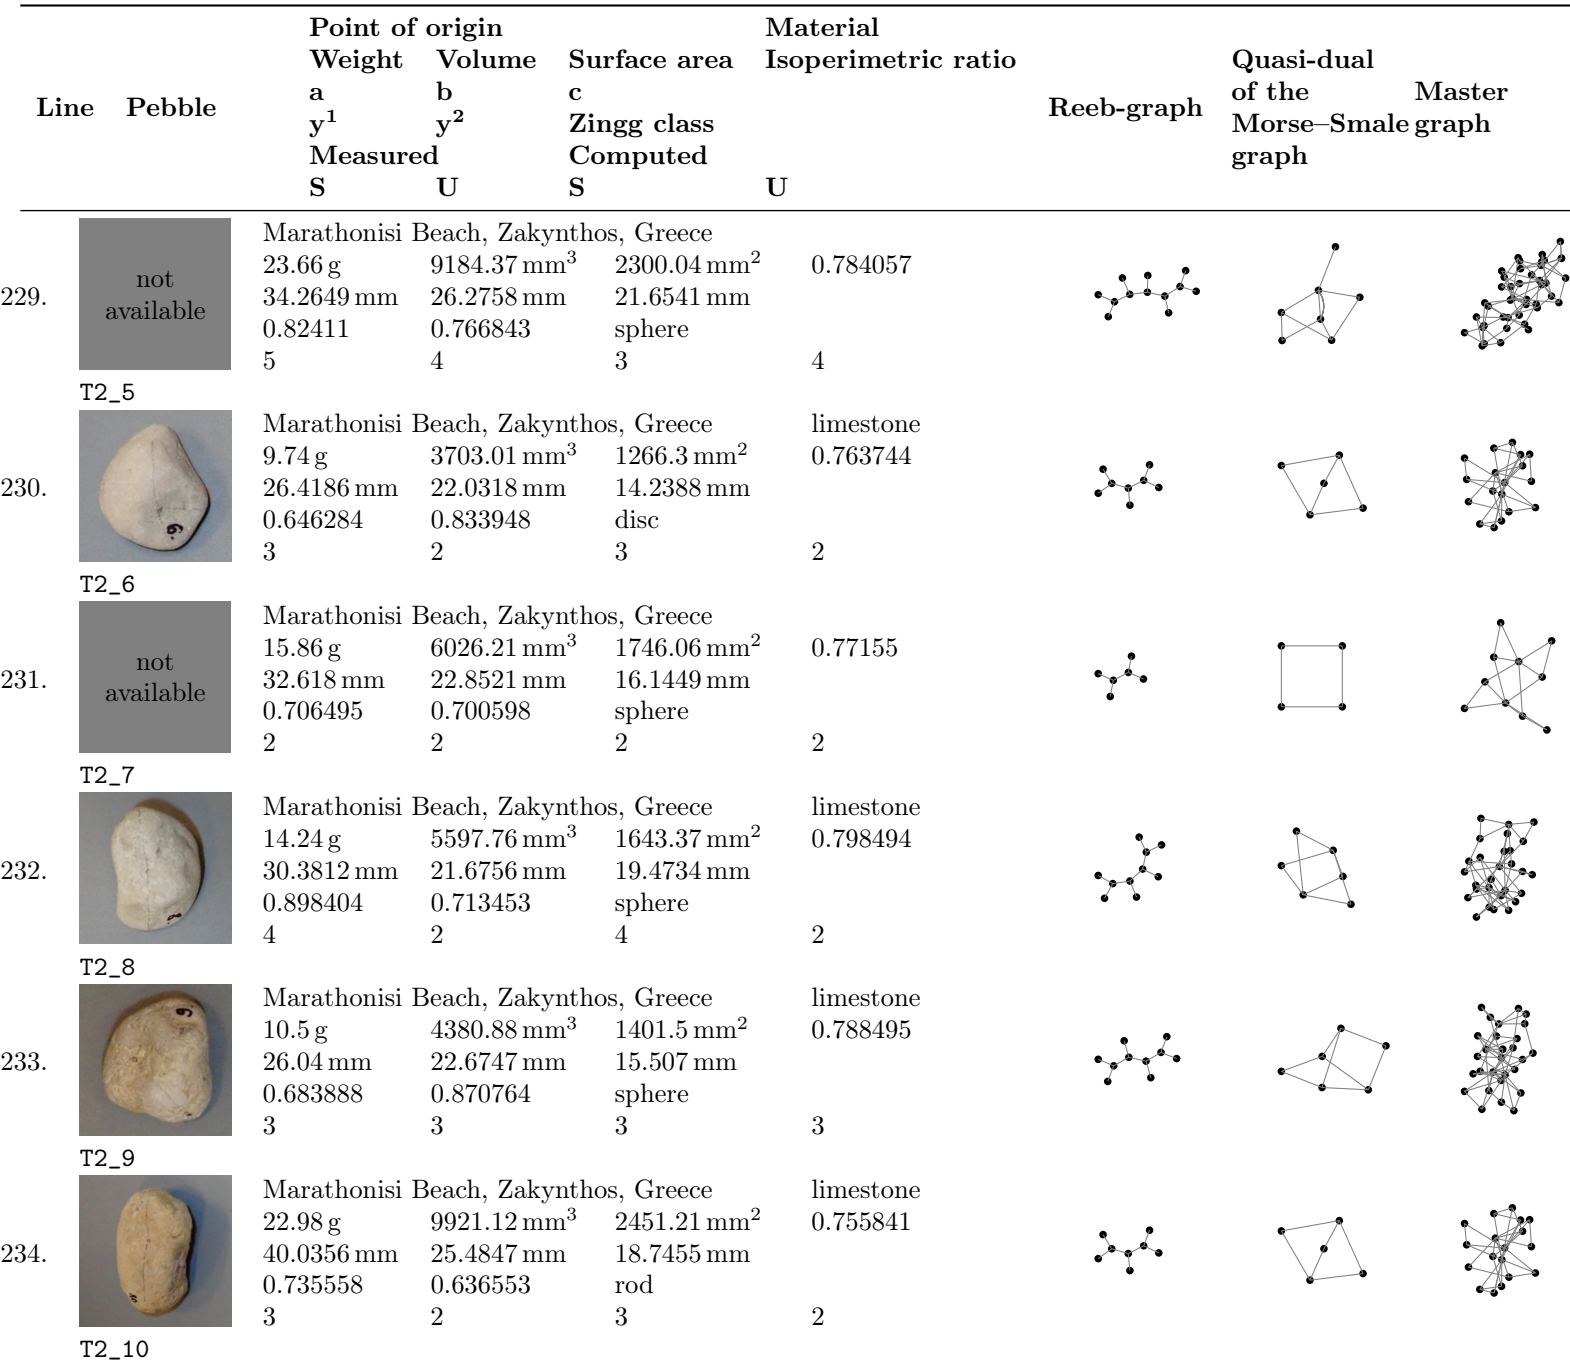   | 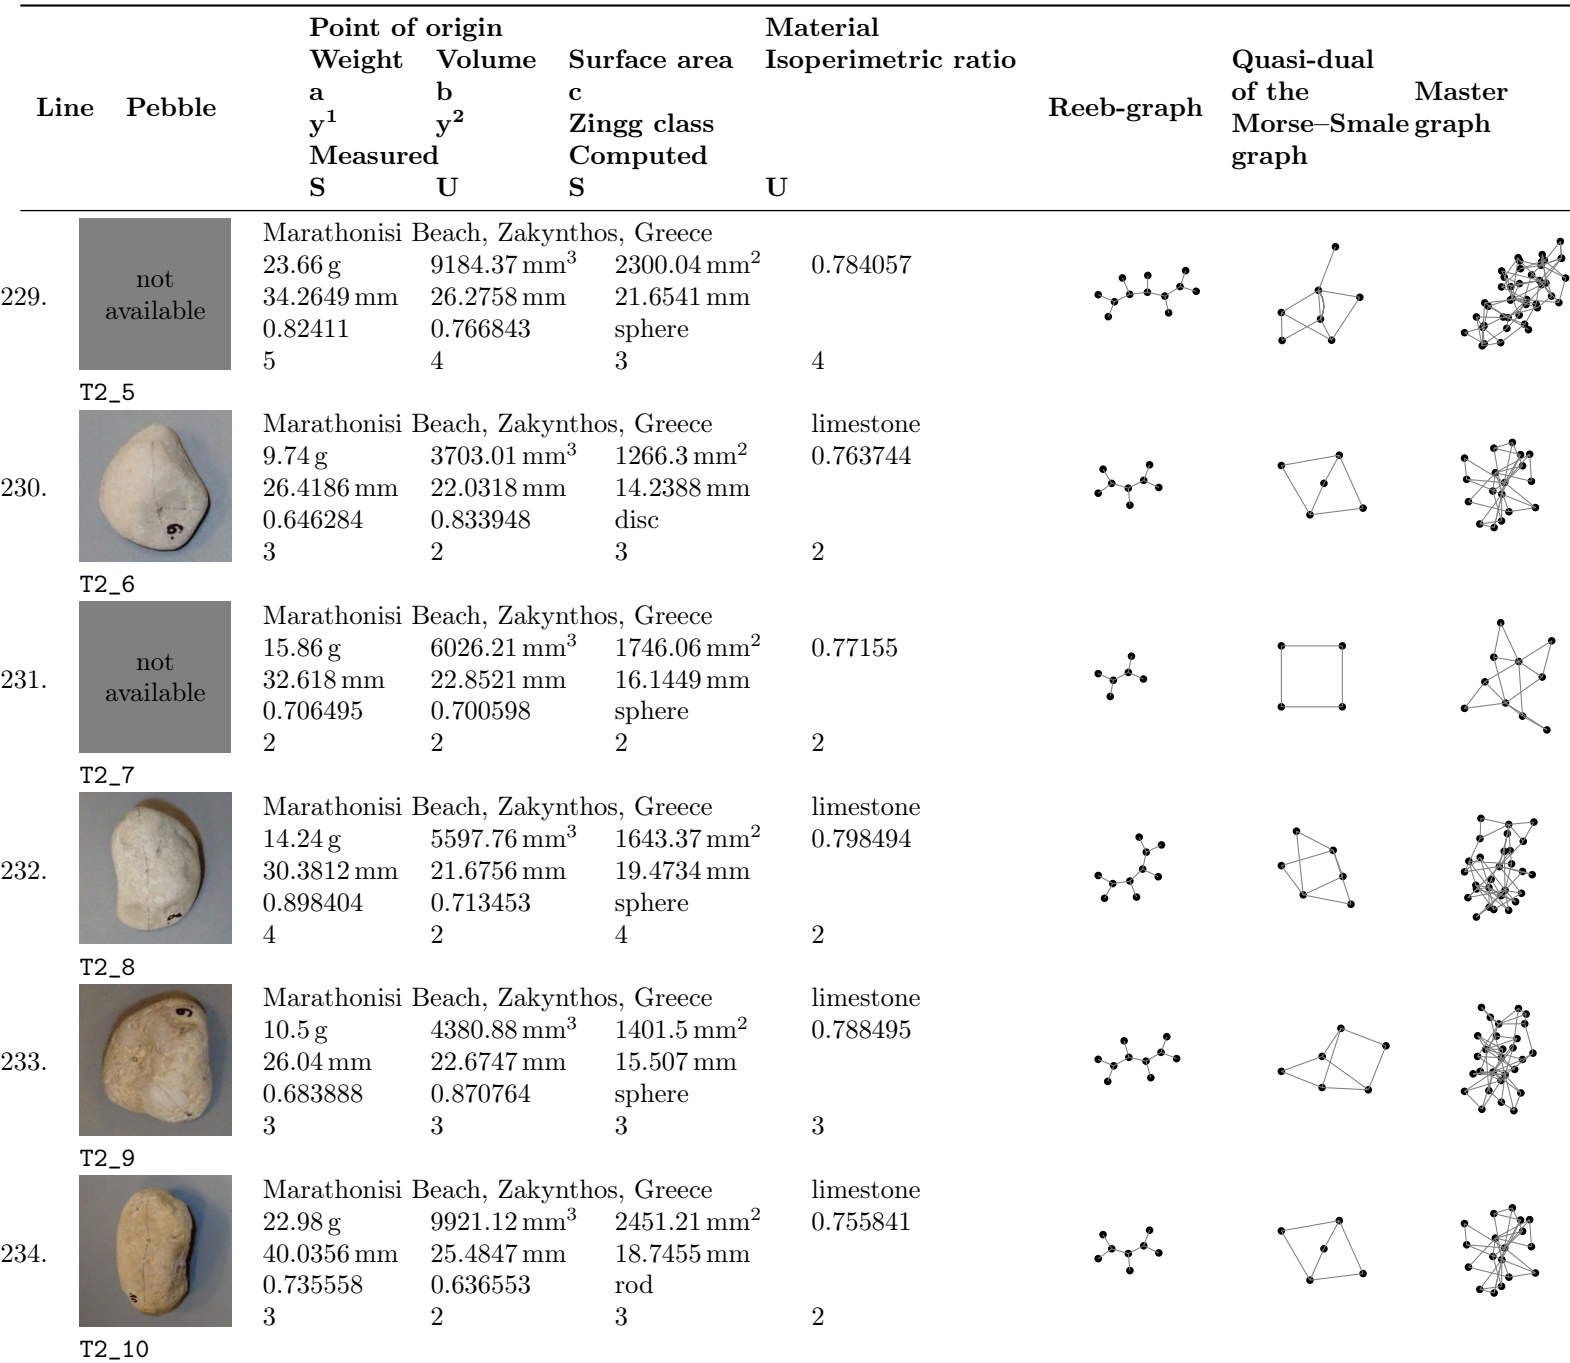   |
|      |                                                                                     | 9.74 g                               | 3703.01 mm <sup>3</sup> | 1266.3 mm <sup>2</sup>       |                       |                                                                                       |                                                                                       |                                                                                       |
|      |                                                                                     | 26.4186 mm                           | 22.0318 mm              | 14.2388 mm                   |                       |                                                                                       |                                                                                       |                                                                                       |
|      |                                                                                     | 0.646284                             | 0.833948                | disc                         |                       |                                                                                       |                                                                                       |                                                                                       |
|      |                                                                                     | 3                                    | 2                       | 3                            |                       |                                                                                       |                                                                                       |                                                                                       |
|      | T2_6                                                                                |                                      |                         |                              | 2                     |                                                                                       |                                                                                       |                                                                                       |
| 231. | 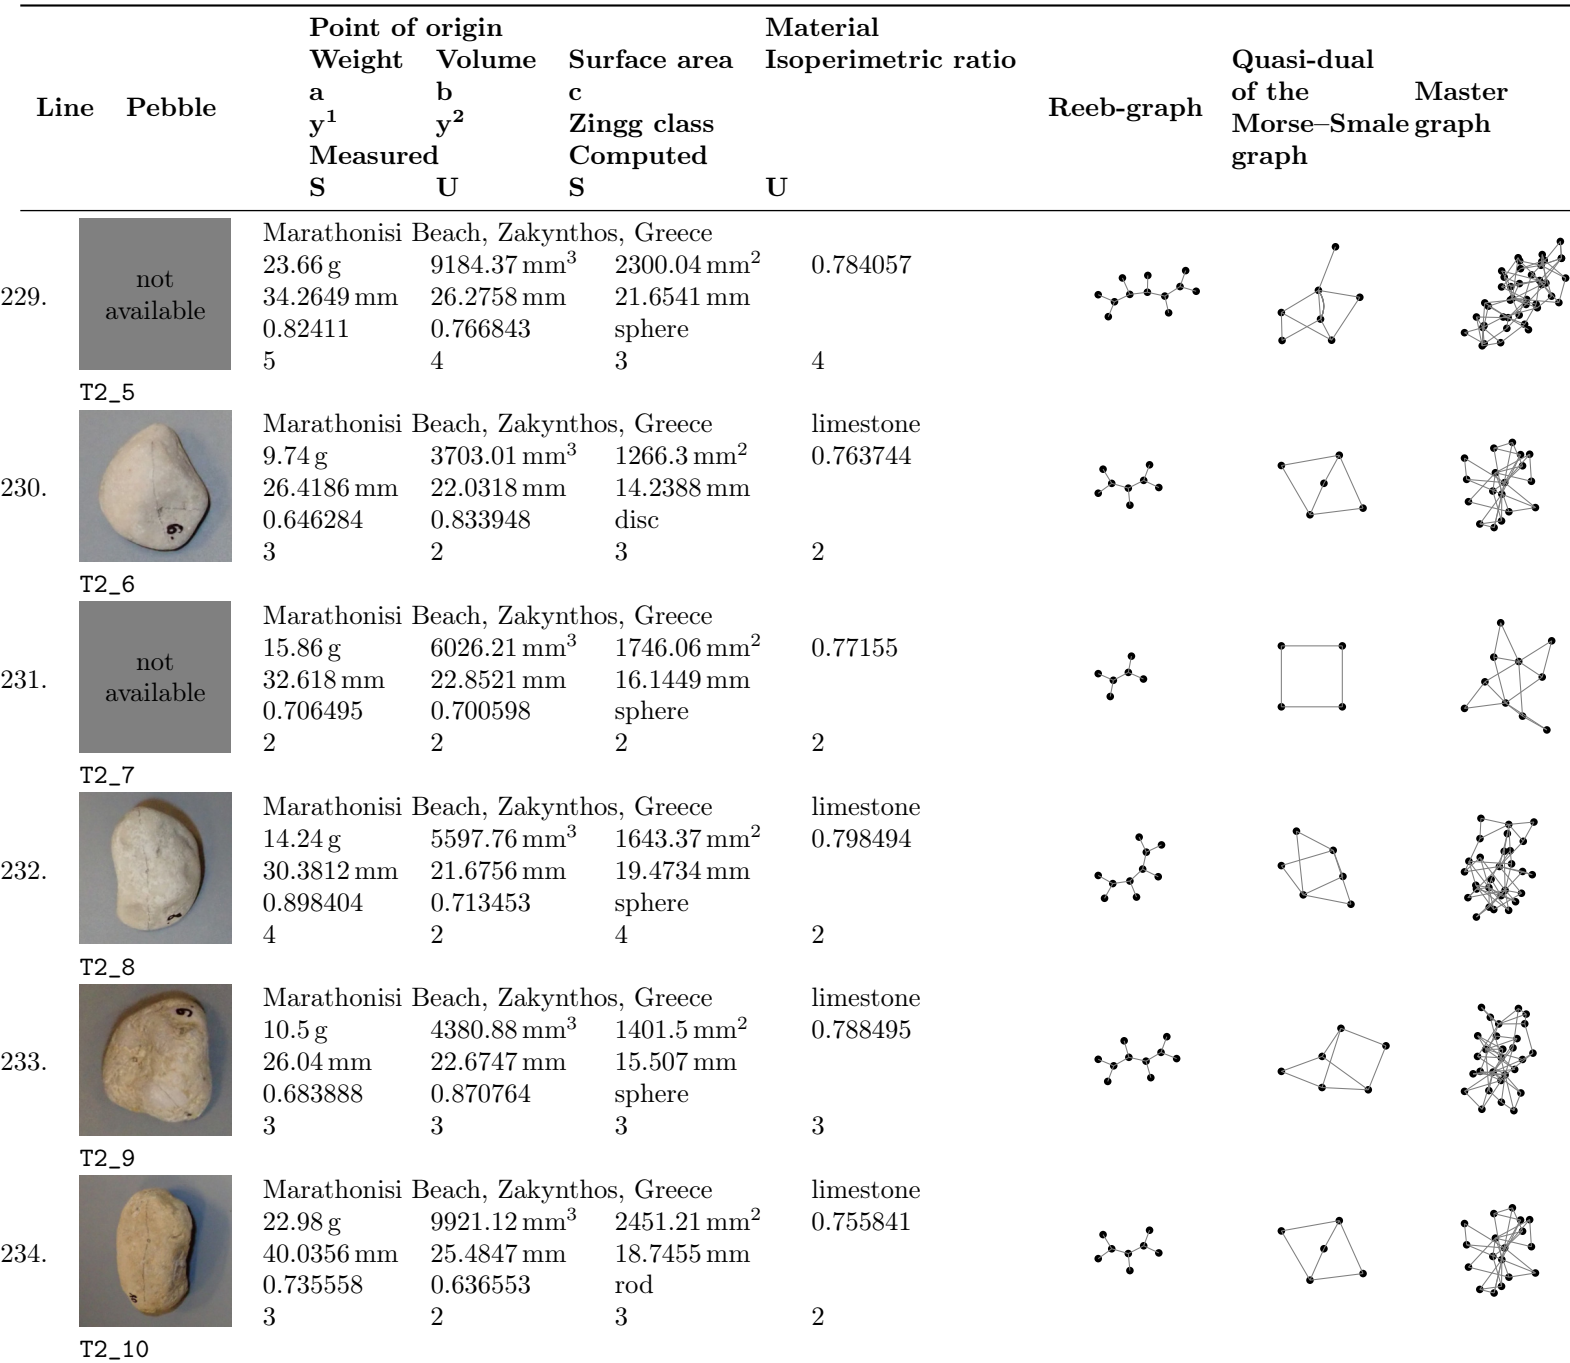   | Marathonisi Beach, Zakynthos, Greece |                         |                              | 0.77155               | 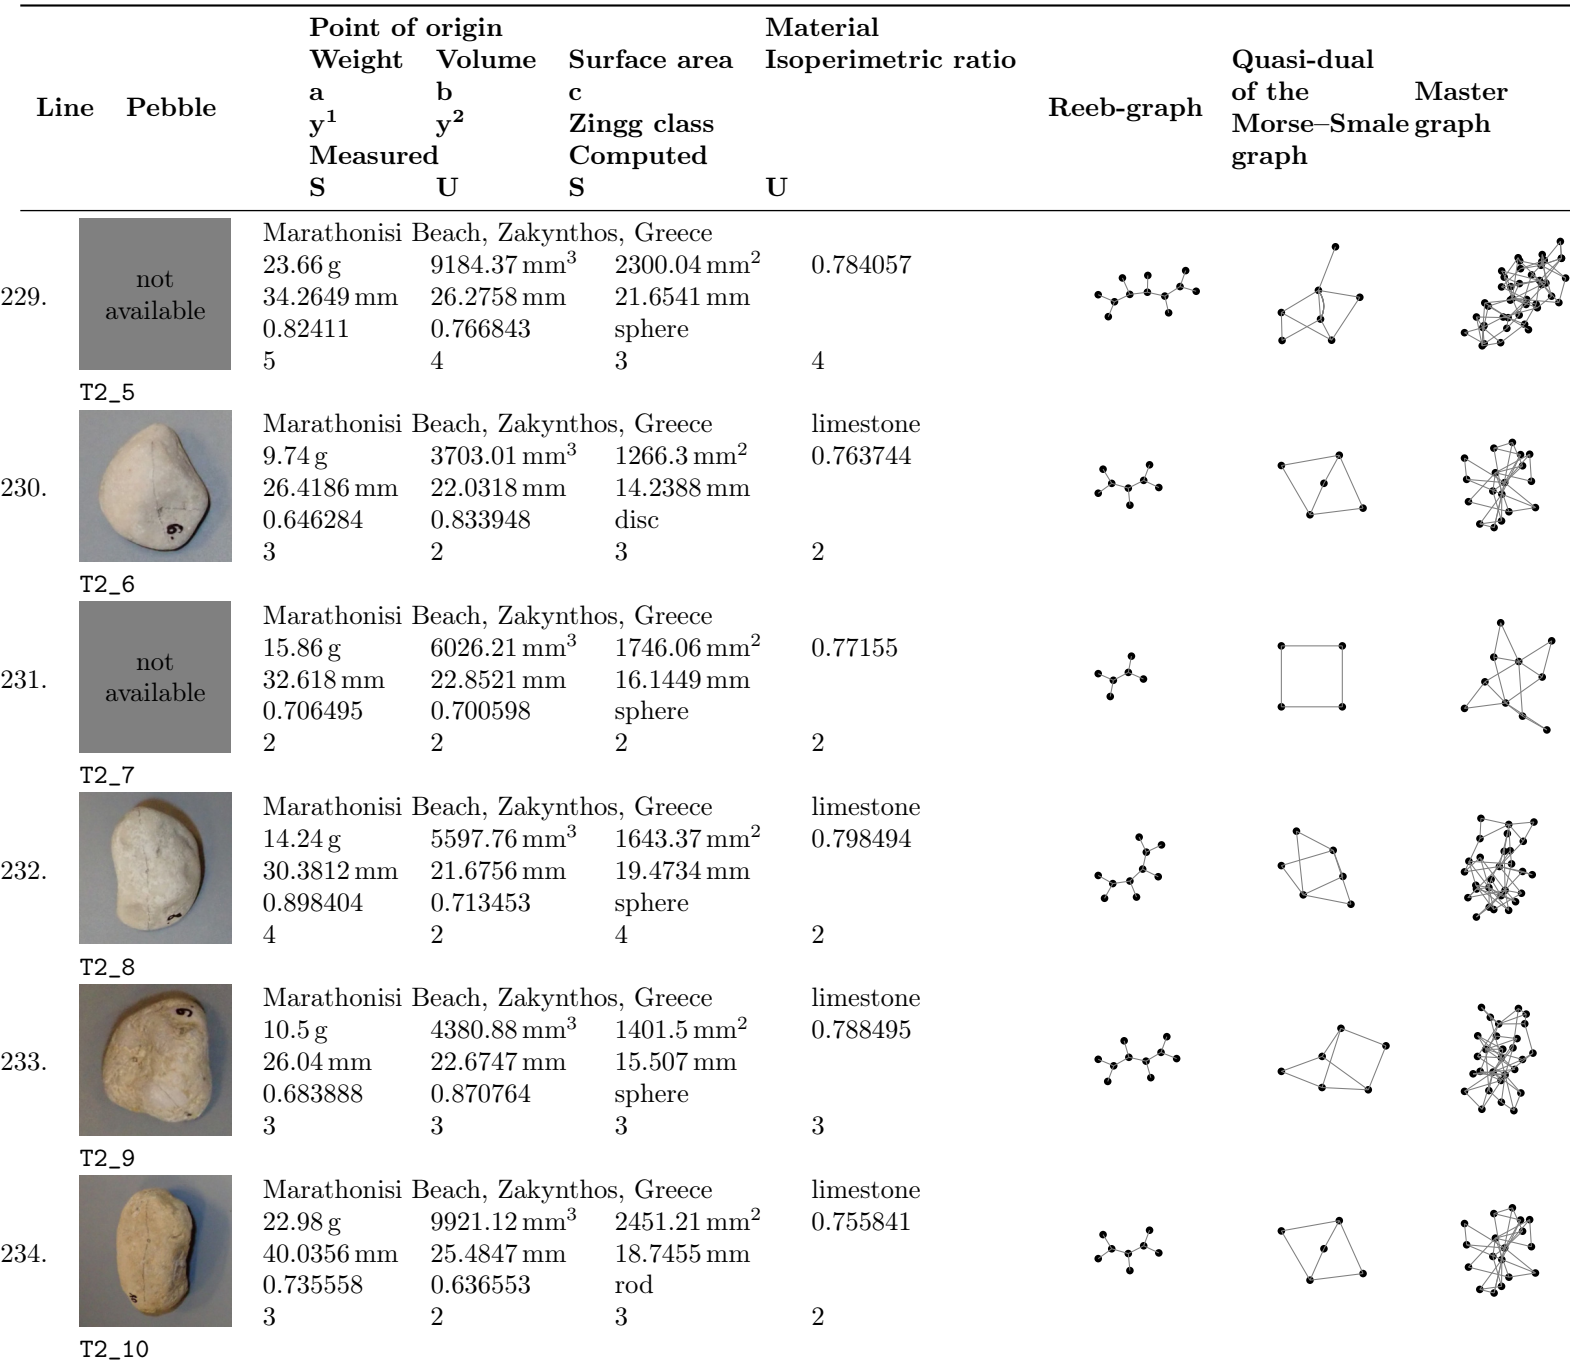   | 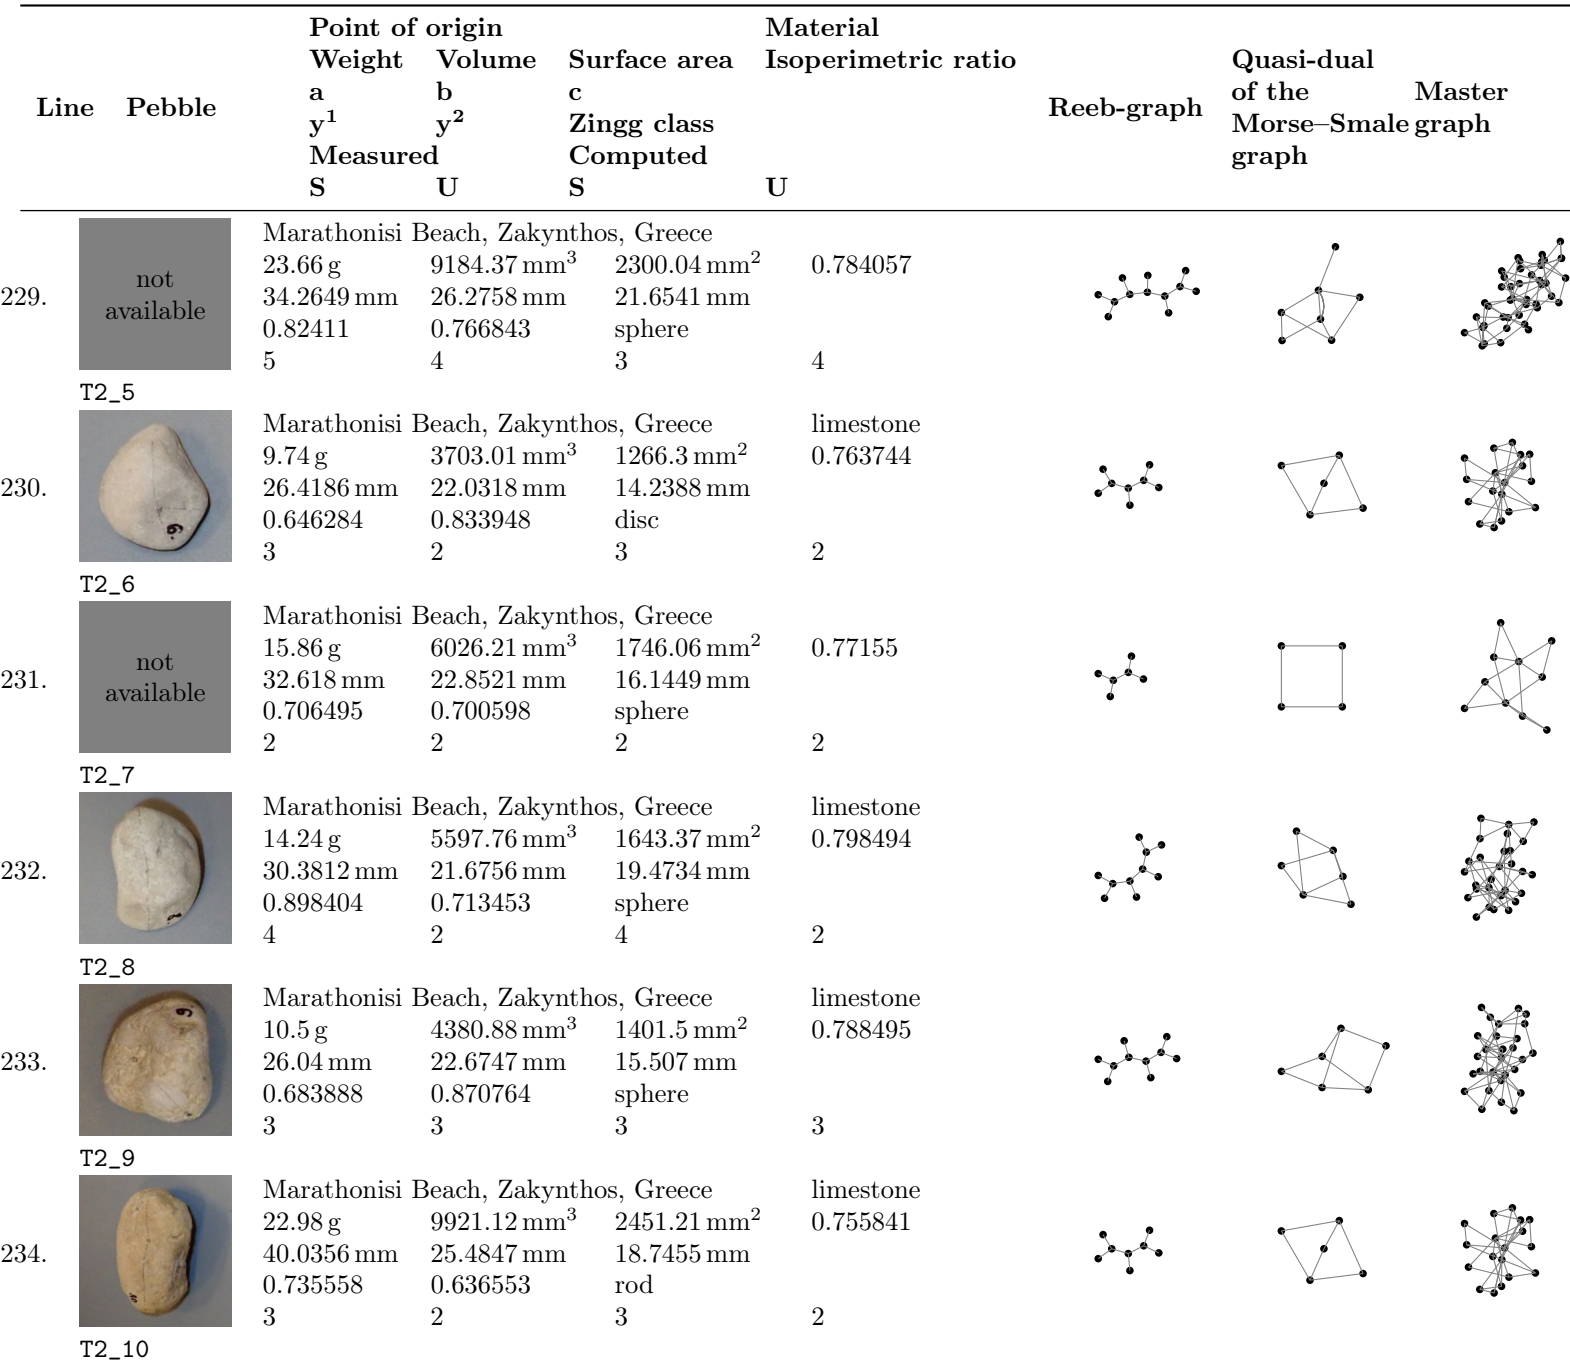   | 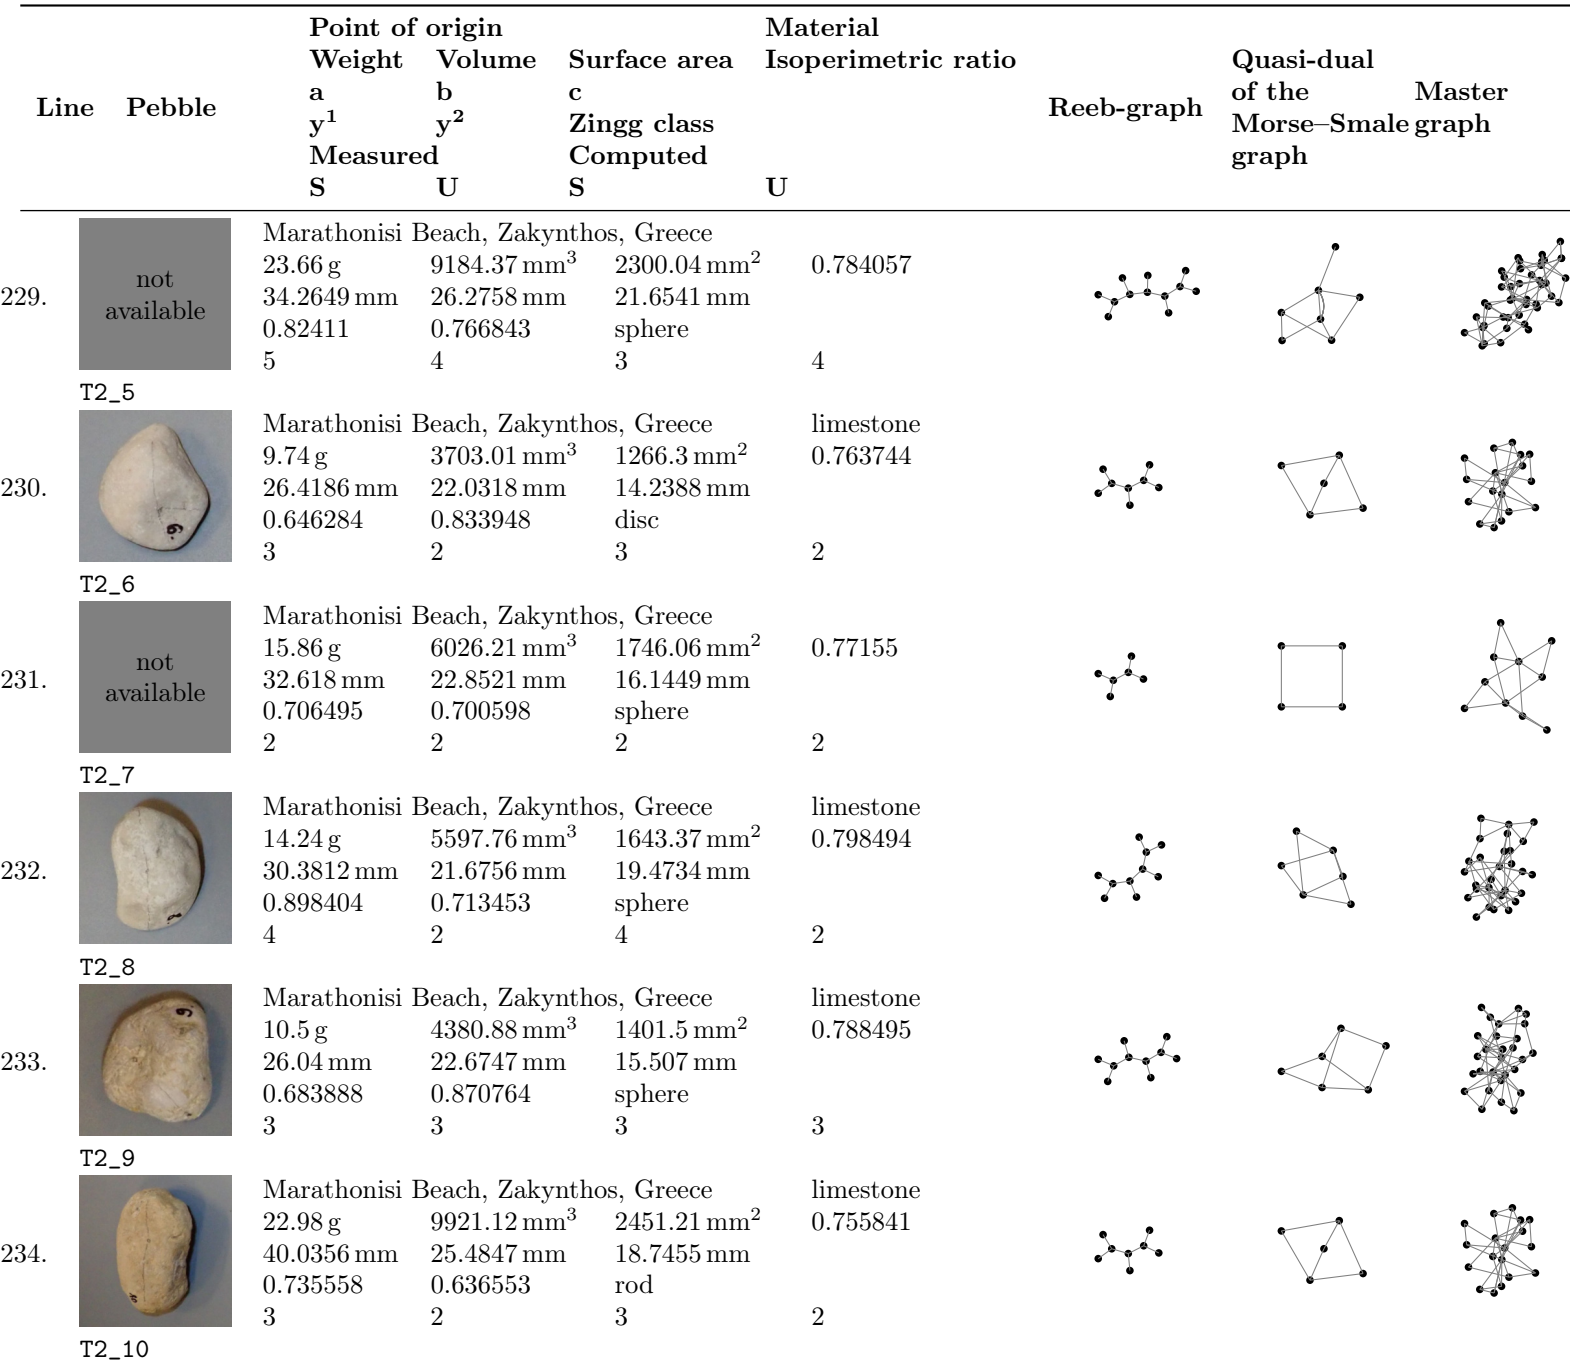   |
|      |                                                                                     | 15.86 g                              | 6026.21 mm <sup>3</sup> | 1746.06 mm <sup>2</sup>      |                       |                                                                                       |                                                                                       |                                                                                       |
|      |                                                                                     | 32.618 mm                            | 22.8521 mm              | 16.1449 mm                   |                       |                                                                                       |                                                                                       |                                                                                       |
|      |                                                                                     | 0.706495                             | 0.700598                | sphere                       |                       |                                                                                       |                                                                                       |                                                                                       |
|      |                                                                                     | 2                                    | 2                       | 2                            |                       |                                                                                       |                                                                                       |                                                                                       |
|      | T2_7                                                                                |                                      |                         |                              | 2                     |                                                                                       |                                                                                       |                                                                                       |
| 232. | 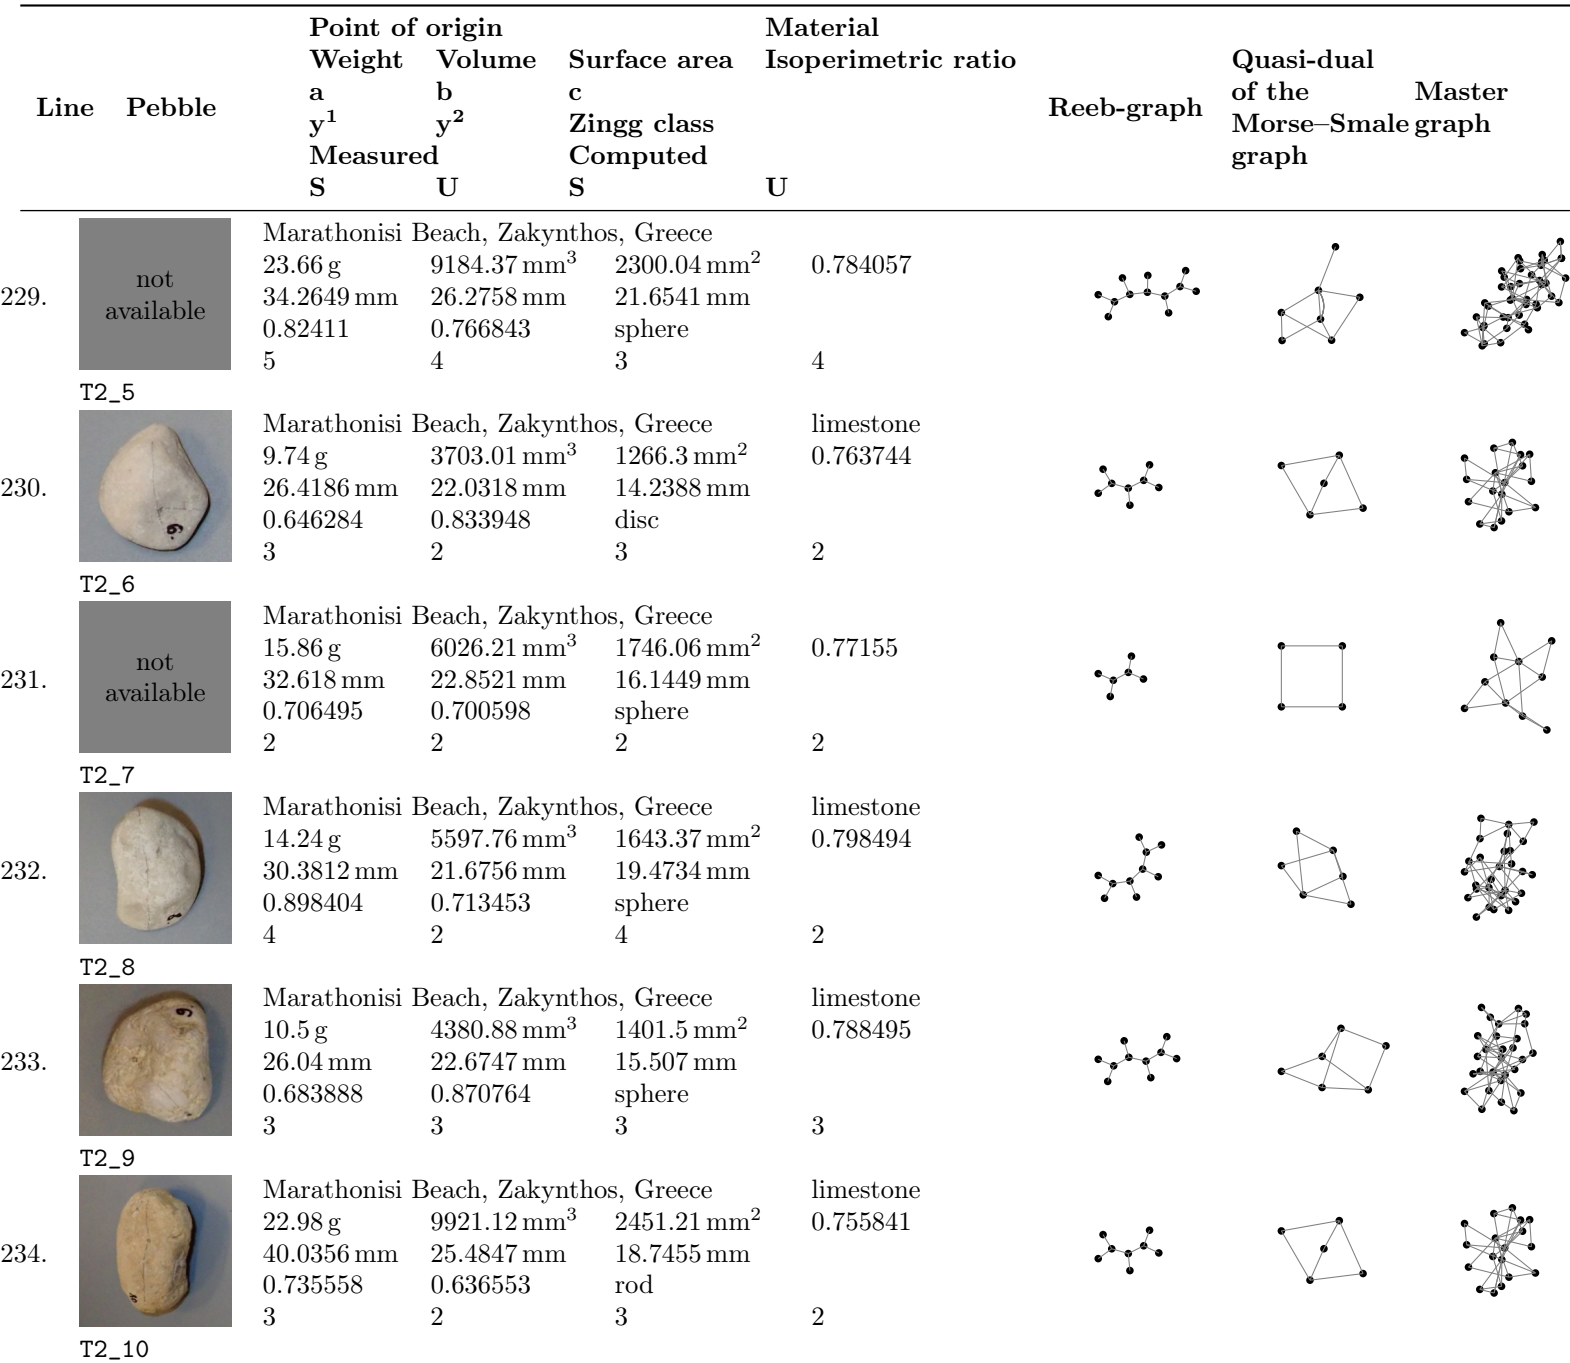  | Marathonisi Beach, Zakynthos, Greece |                         |                              | limestone<br>0.798494 | 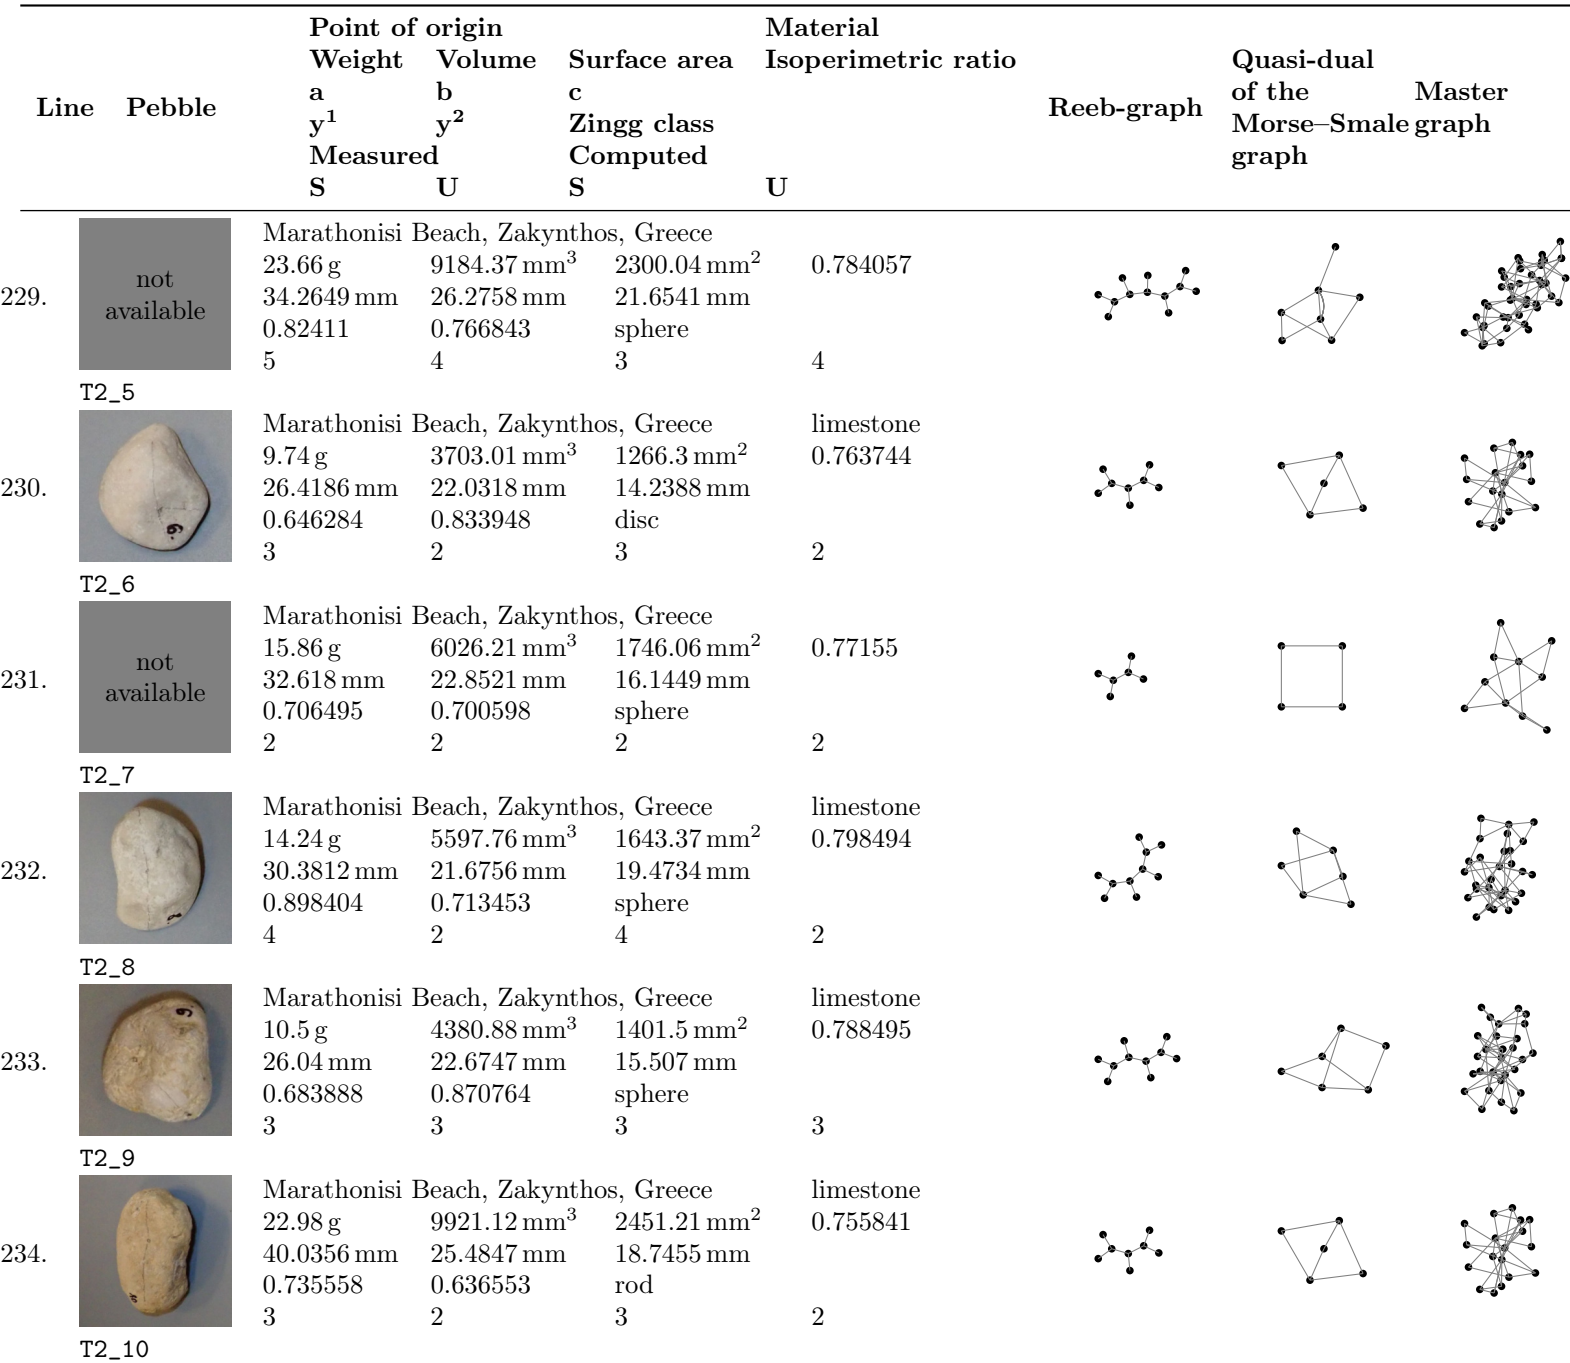  | 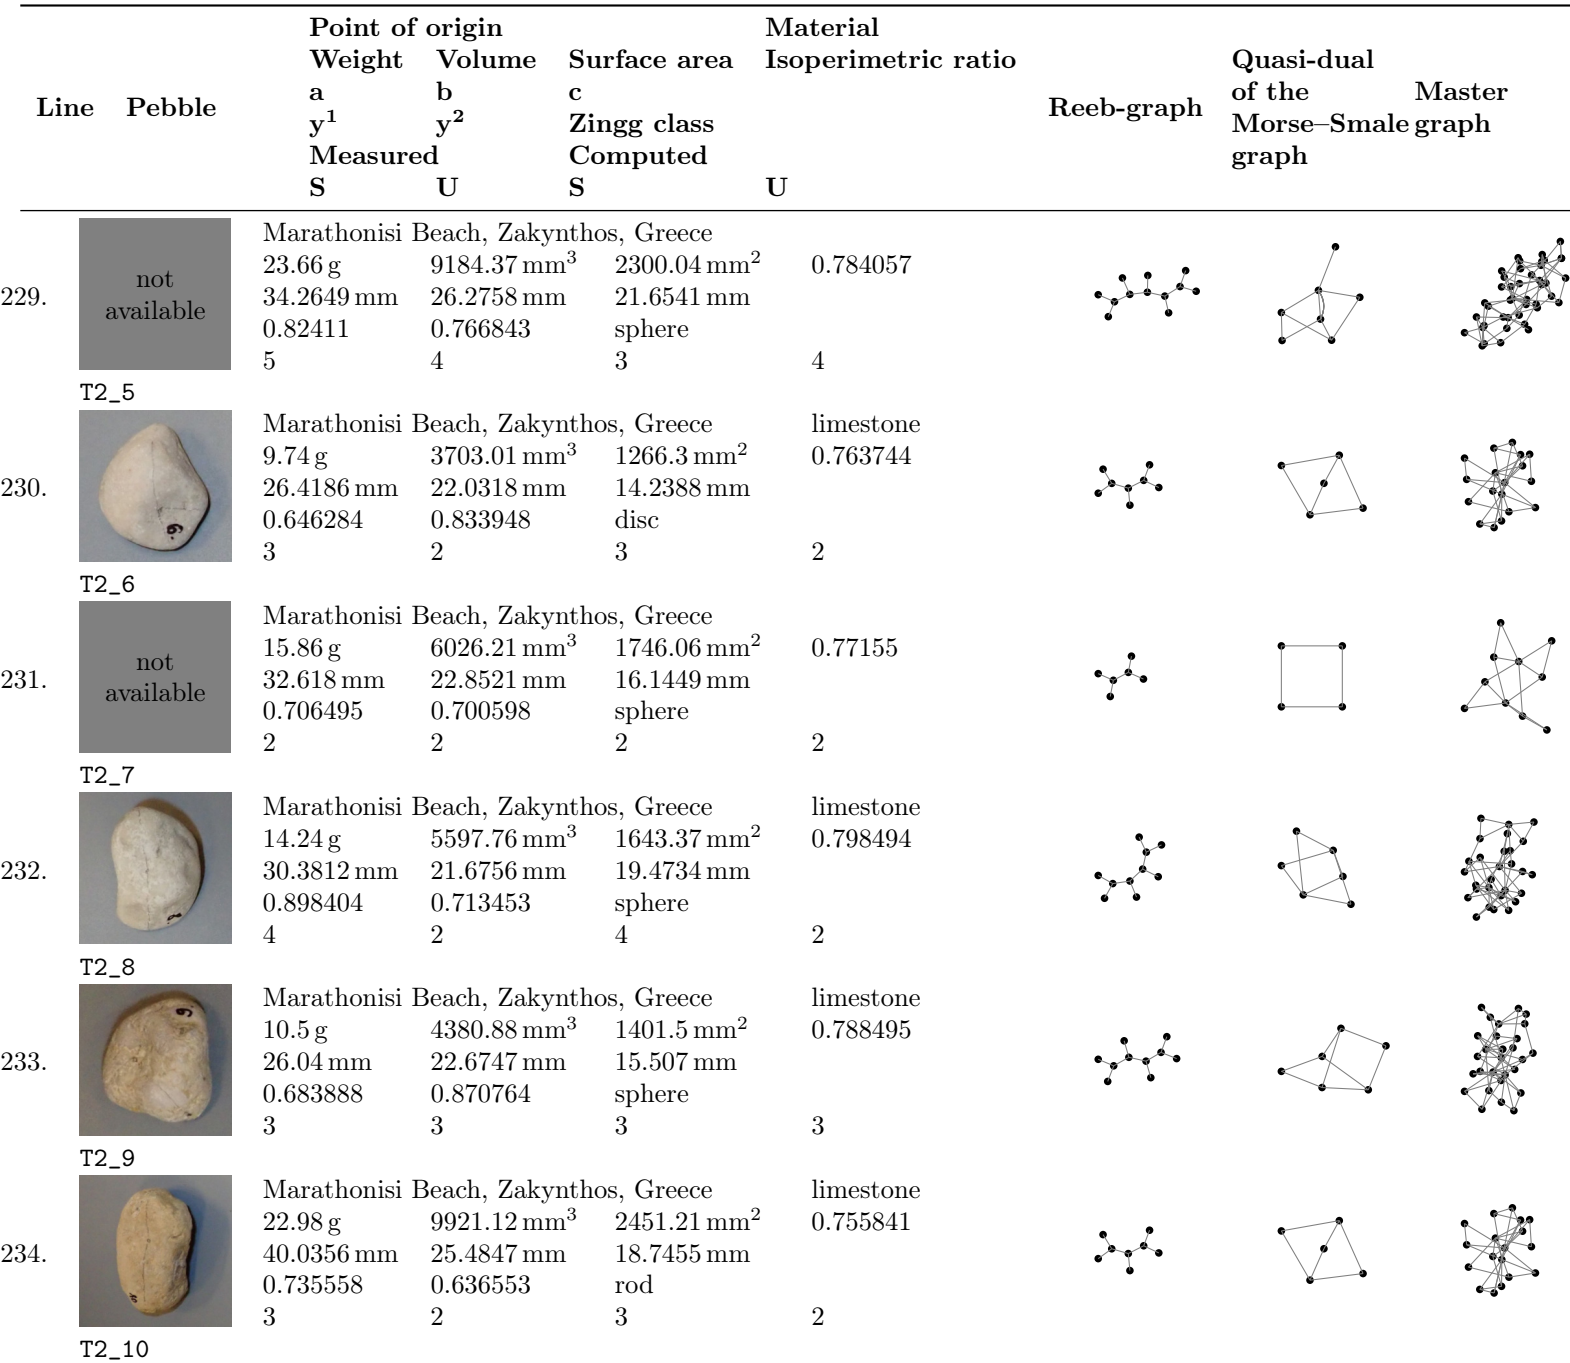  | 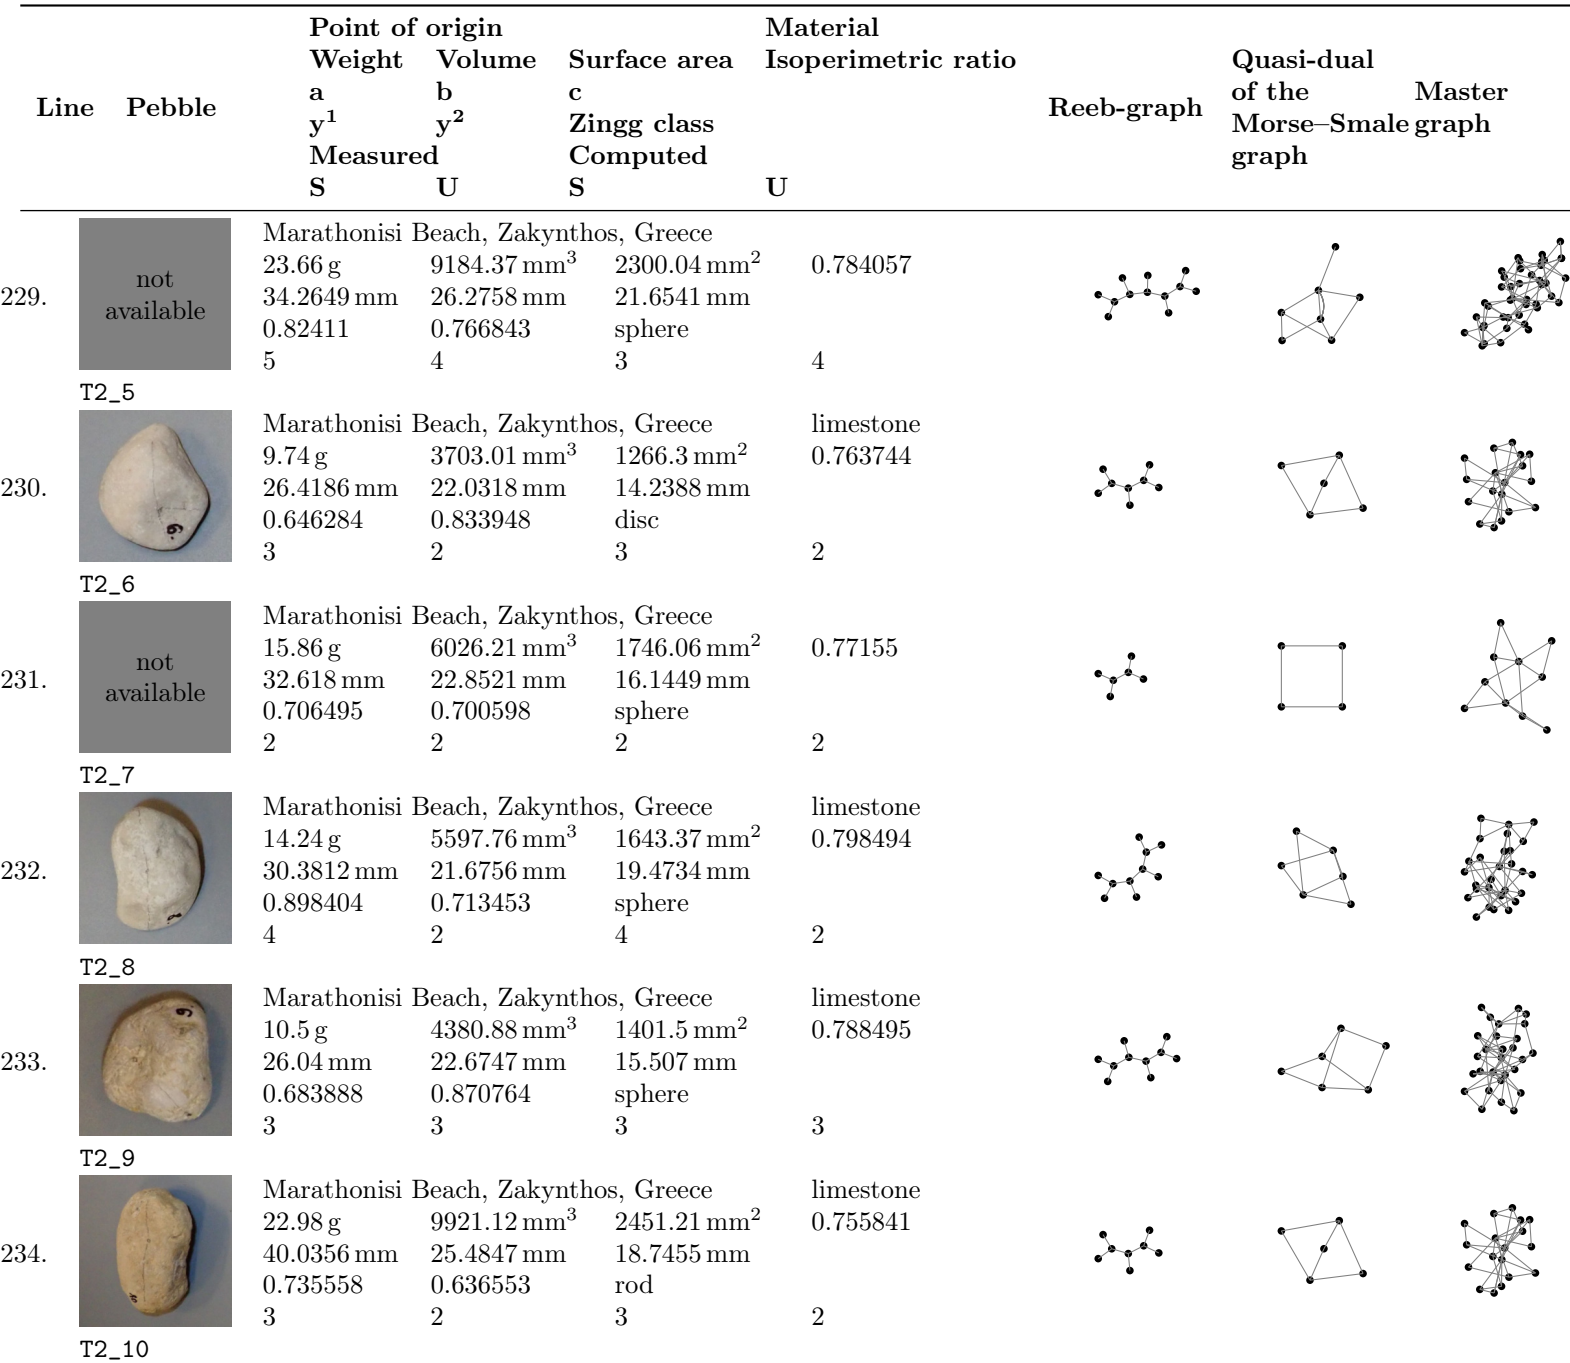  |
|      |                                                                                     | 14.24 g                              | 5597.76 mm <sup>3</sup> | 1643.37 mm <sup>2</sup>      |                       |                                                                                       |                                                                                       |                                                                                       |
|      |                                                                                     | 30.3812 mm                           | 21.6756 mm              | 19.4734 mm                   |                       |                                                                                       |                                                                                       |                                                                                       |
|      |                                                                                     | 0.898404                             | 0.713453                | sphere                       |                       |                                                                                       |                                                                                       |                                                                                       |
|      |                                                                                     | 4                                    | 2                       | 4                            |                       |                                                                                       |                                                                                       |                                                                                       |
|      | T2_8                                                                                |                                      |                         |                              | 2                     |                                                                                       |                                                                                       |                                                                                       |
| 233. | 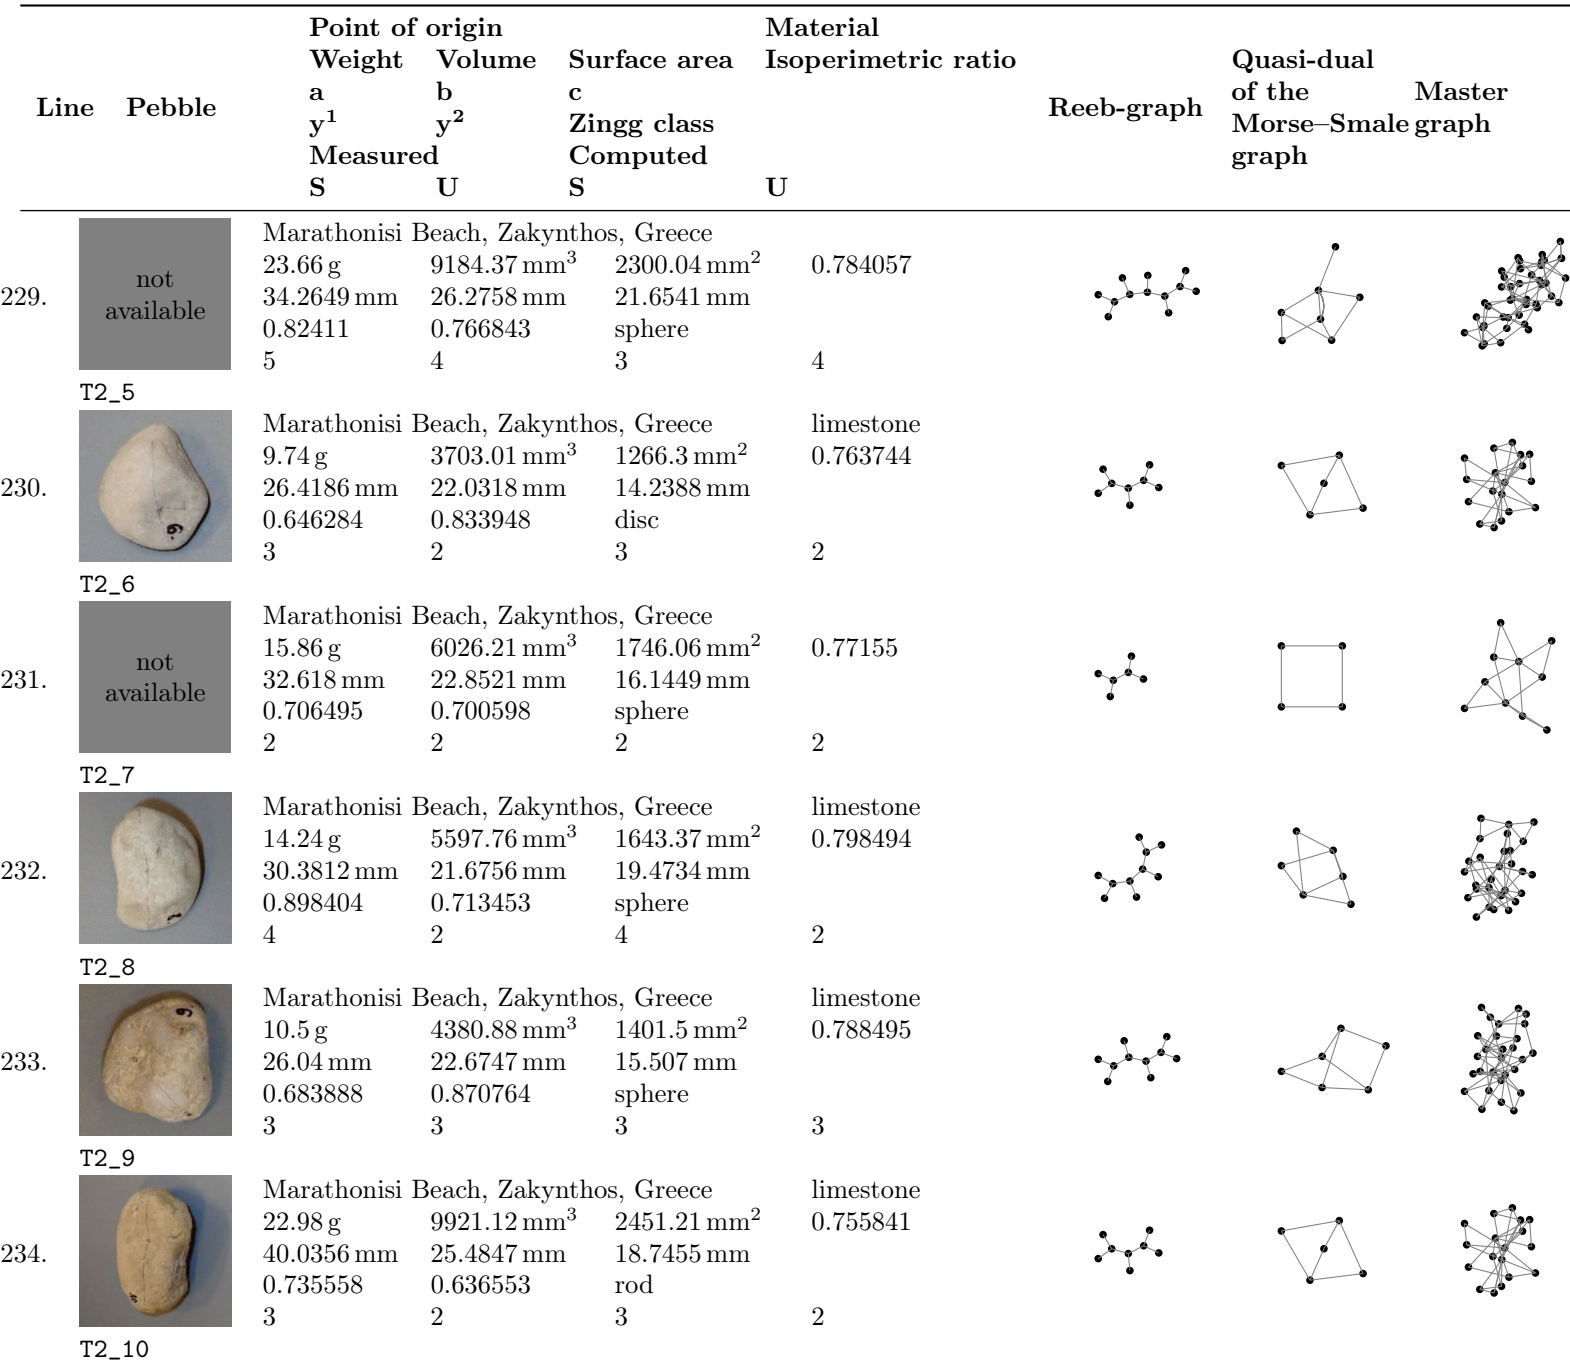 | Marathonisi Beach, Zakynthos, Greece |                         |                              | limestone<br>0.788495 | 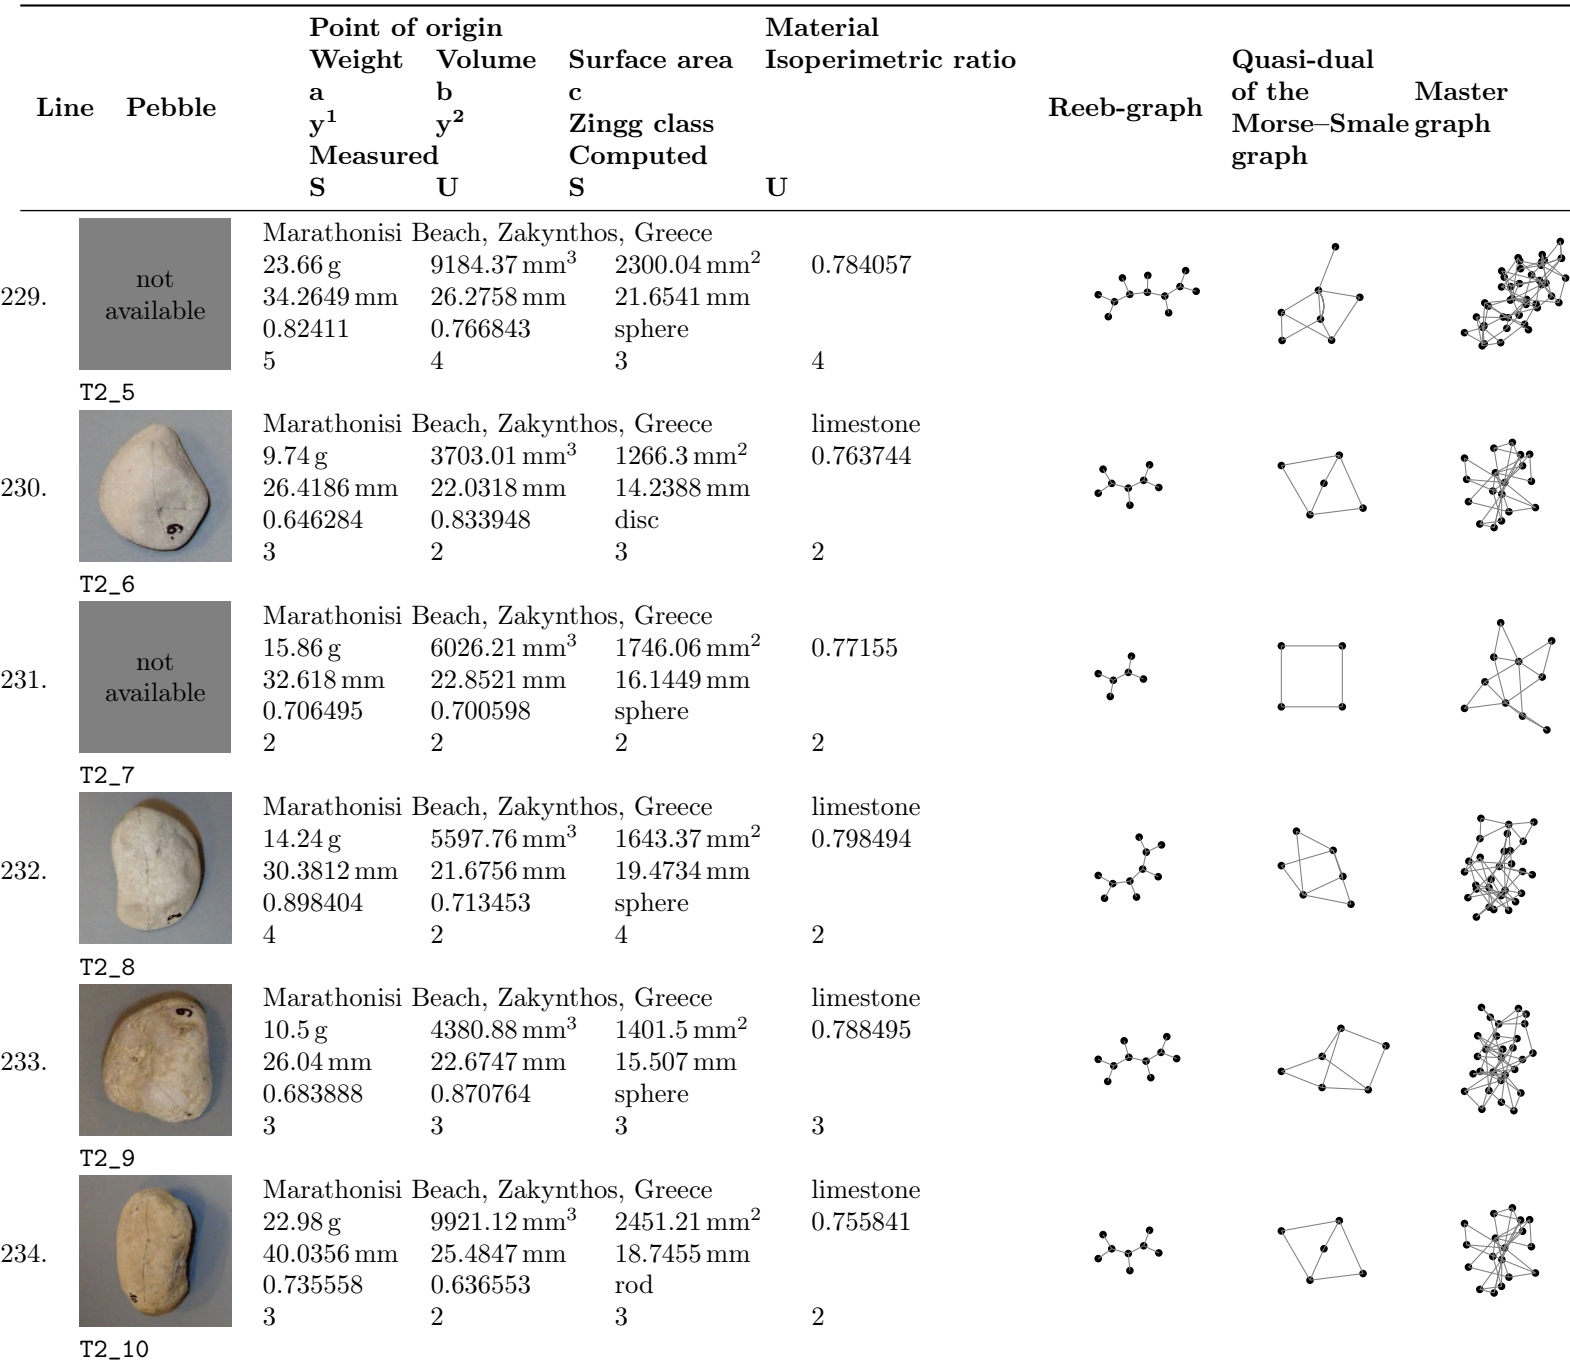 | 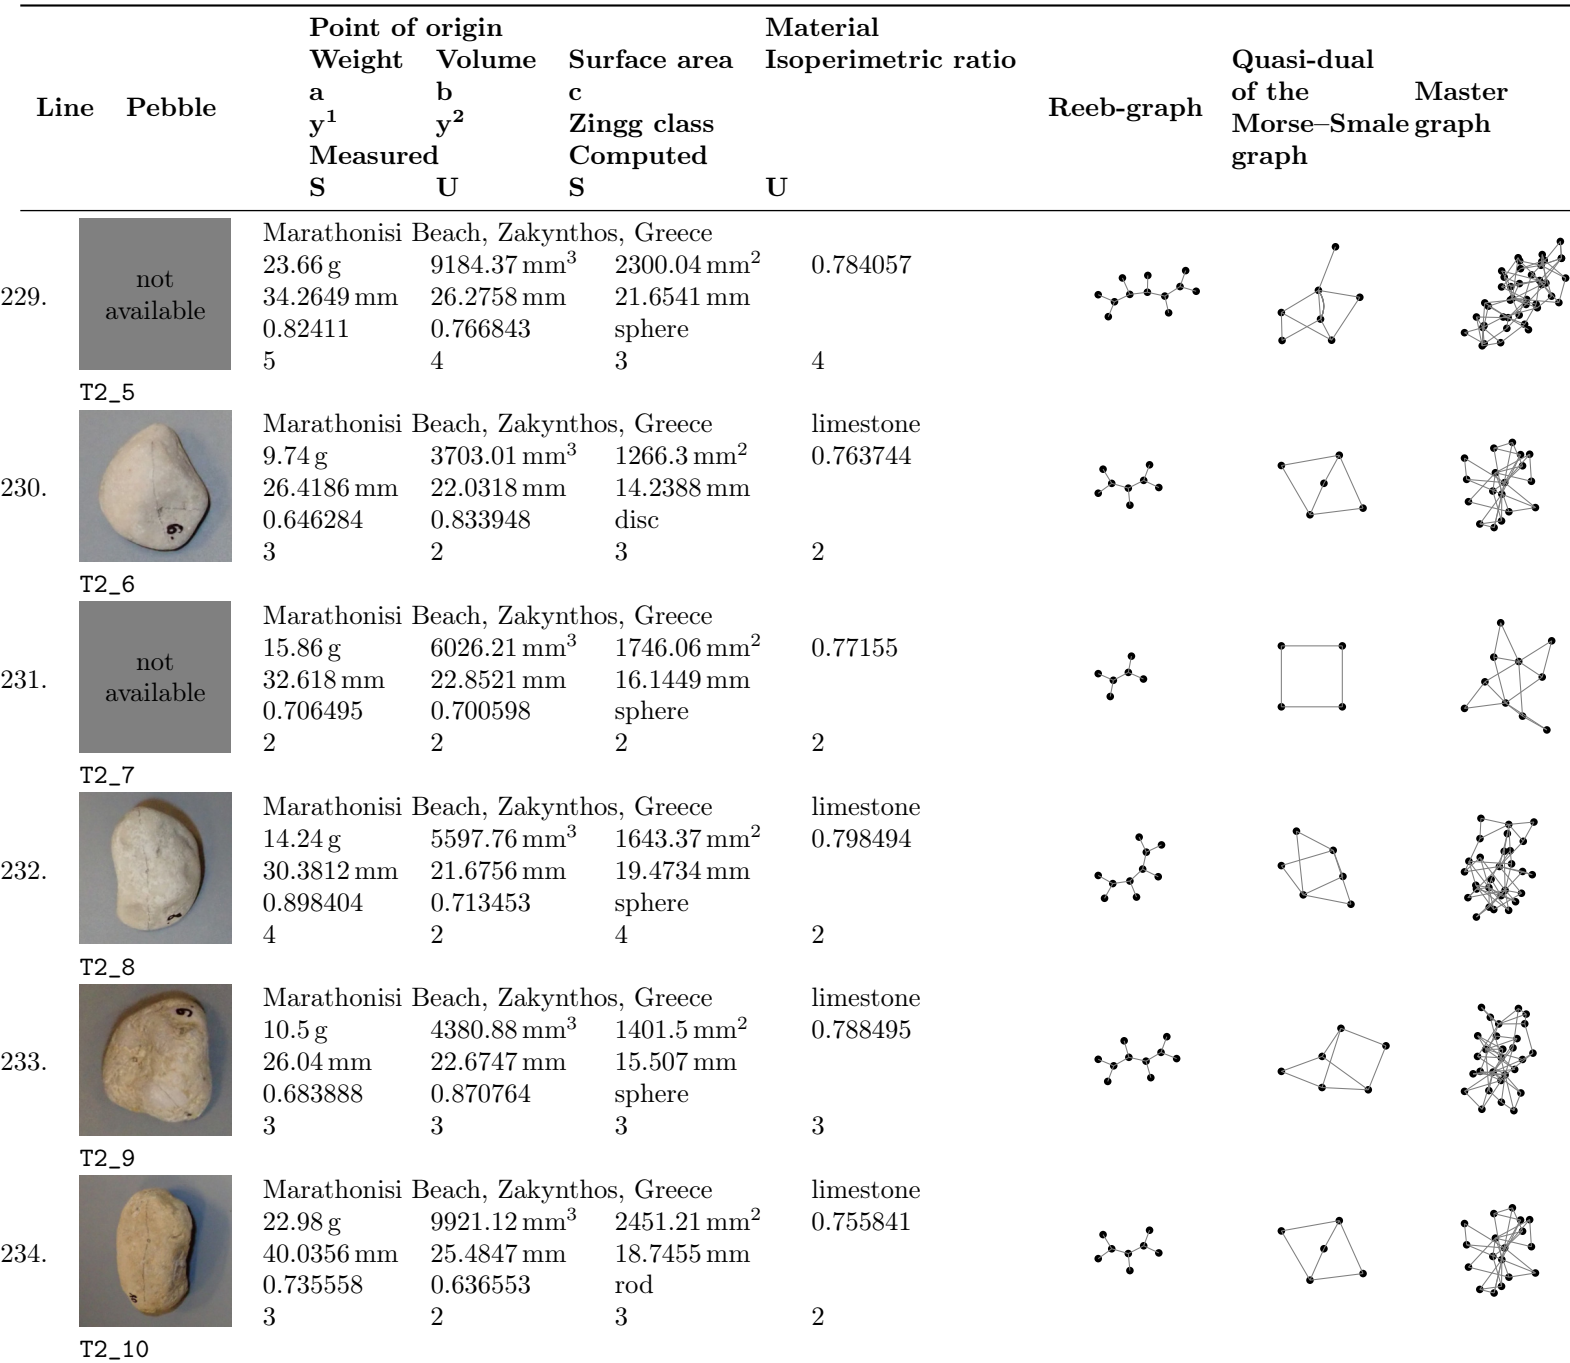 | 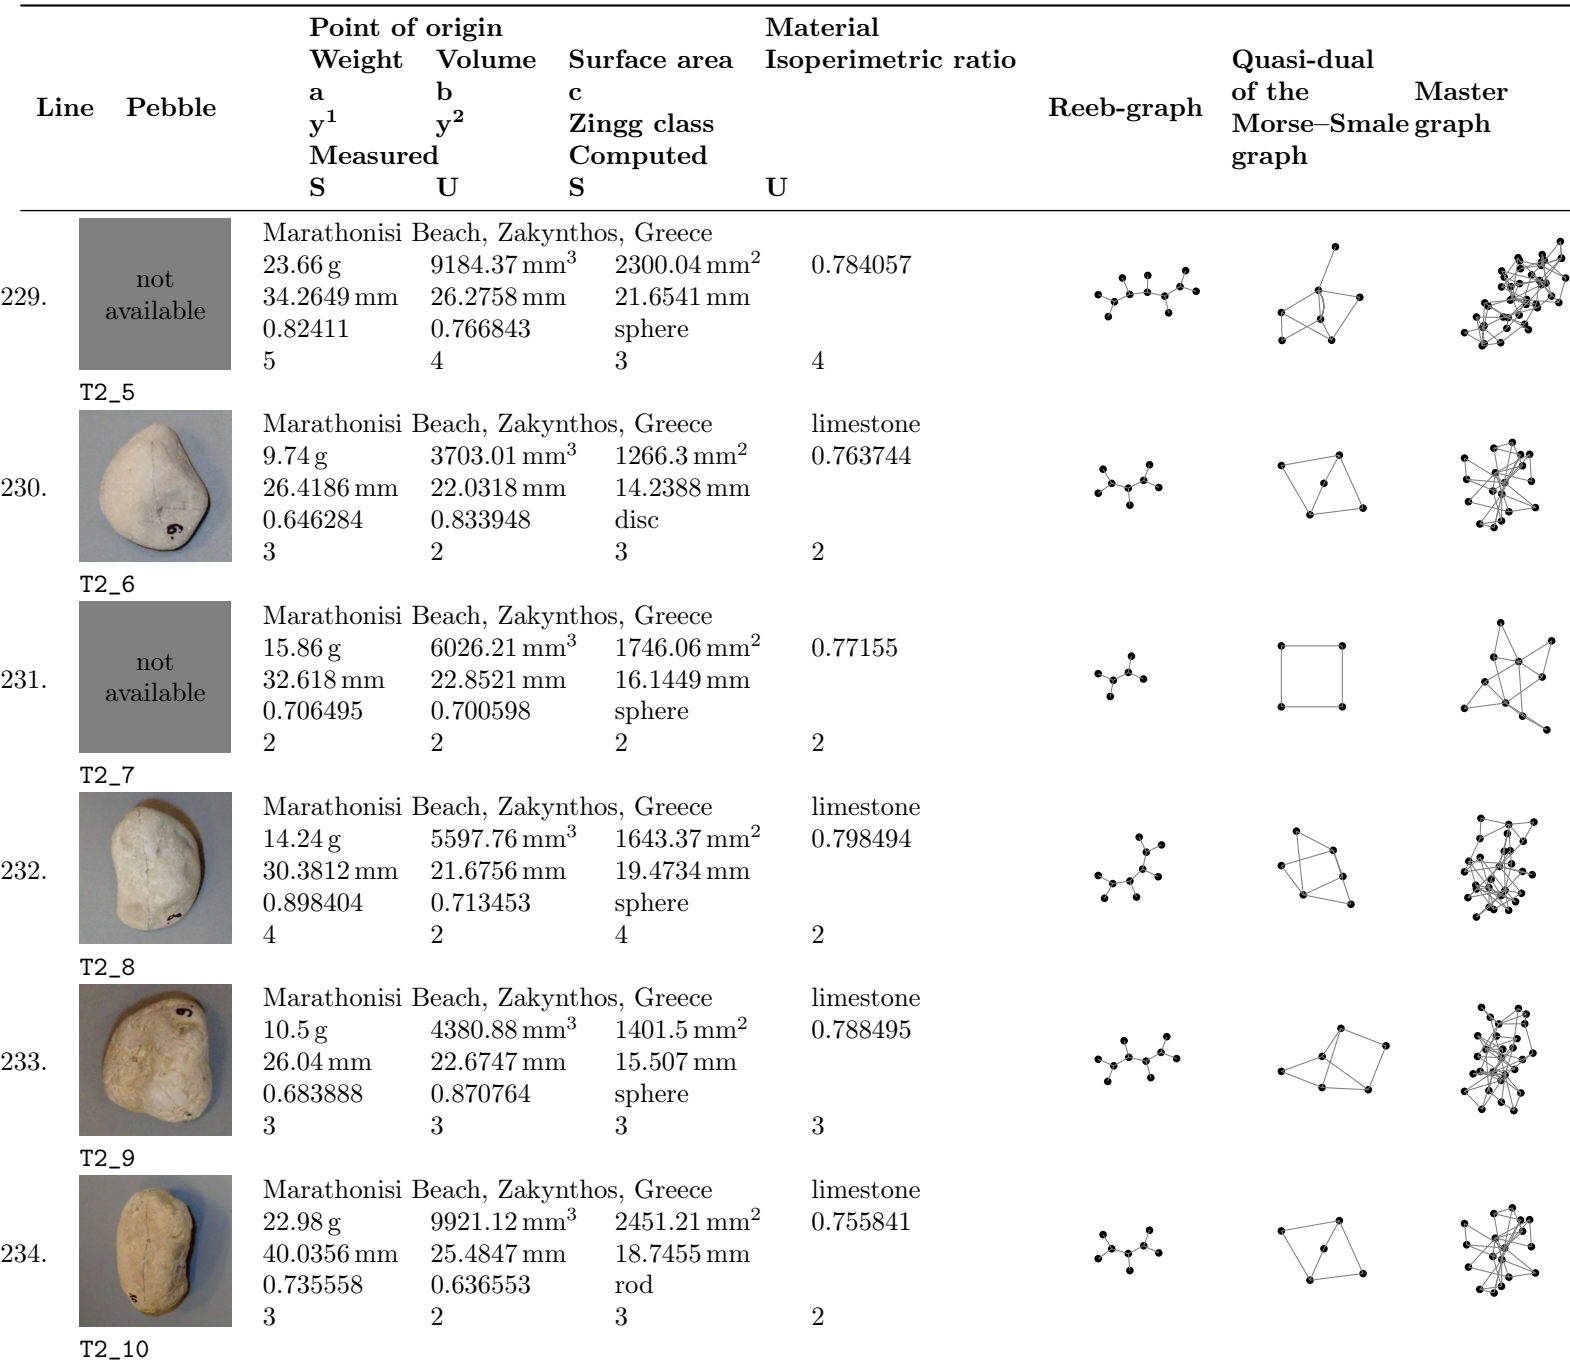 |
|      |                                                                                     | 10.5 g                               | 4380.88 mm <sup>3</sup> | 1401.5 mm <sup>2</sup>       |                       |                                                                                       |                                                                                       |                                                                                       |
|      |                                                                                     | 26.04 mm                             | 22.6747 mm              | 15.507 mm                    |                       |                                                                                       |                                                                                       |                                                                                       |
|      |                                                                                     | 0.683888                             | 0.870764                | sphere                       |                       |                                                                                       |                                                                                       |                                                                                       |
|      |                                                                                     | 3                                    | 3                       | 3                            |                       |                                                                                       |                                                                                       |                                                                                       |
|      | T2_9                                                                                |                                      |                         |                              | 3                     |                                                                                       |                                                                                       |                                                                                       |
| 234. | 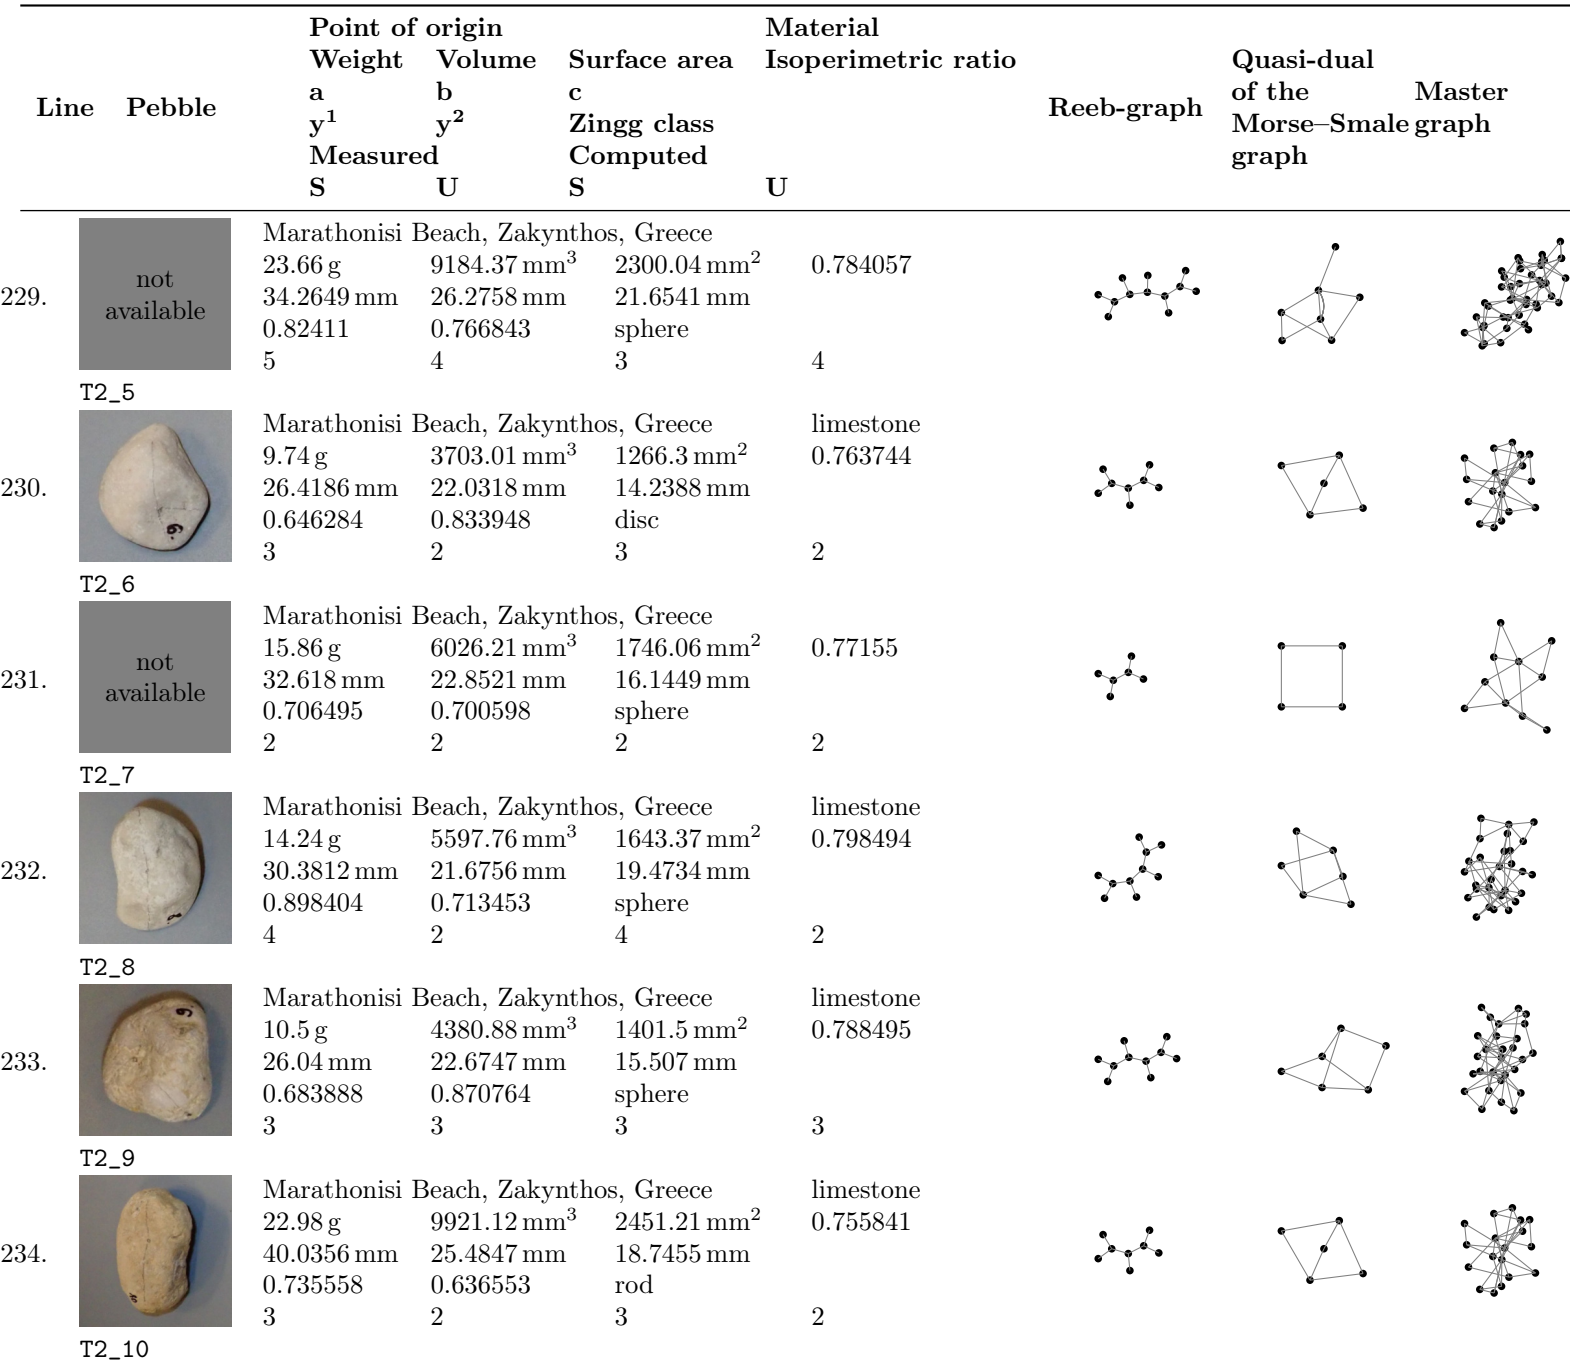 | Marathonisi Beach, Zakynthos, Greece |                         |                              | limestone<br>0.755841 | 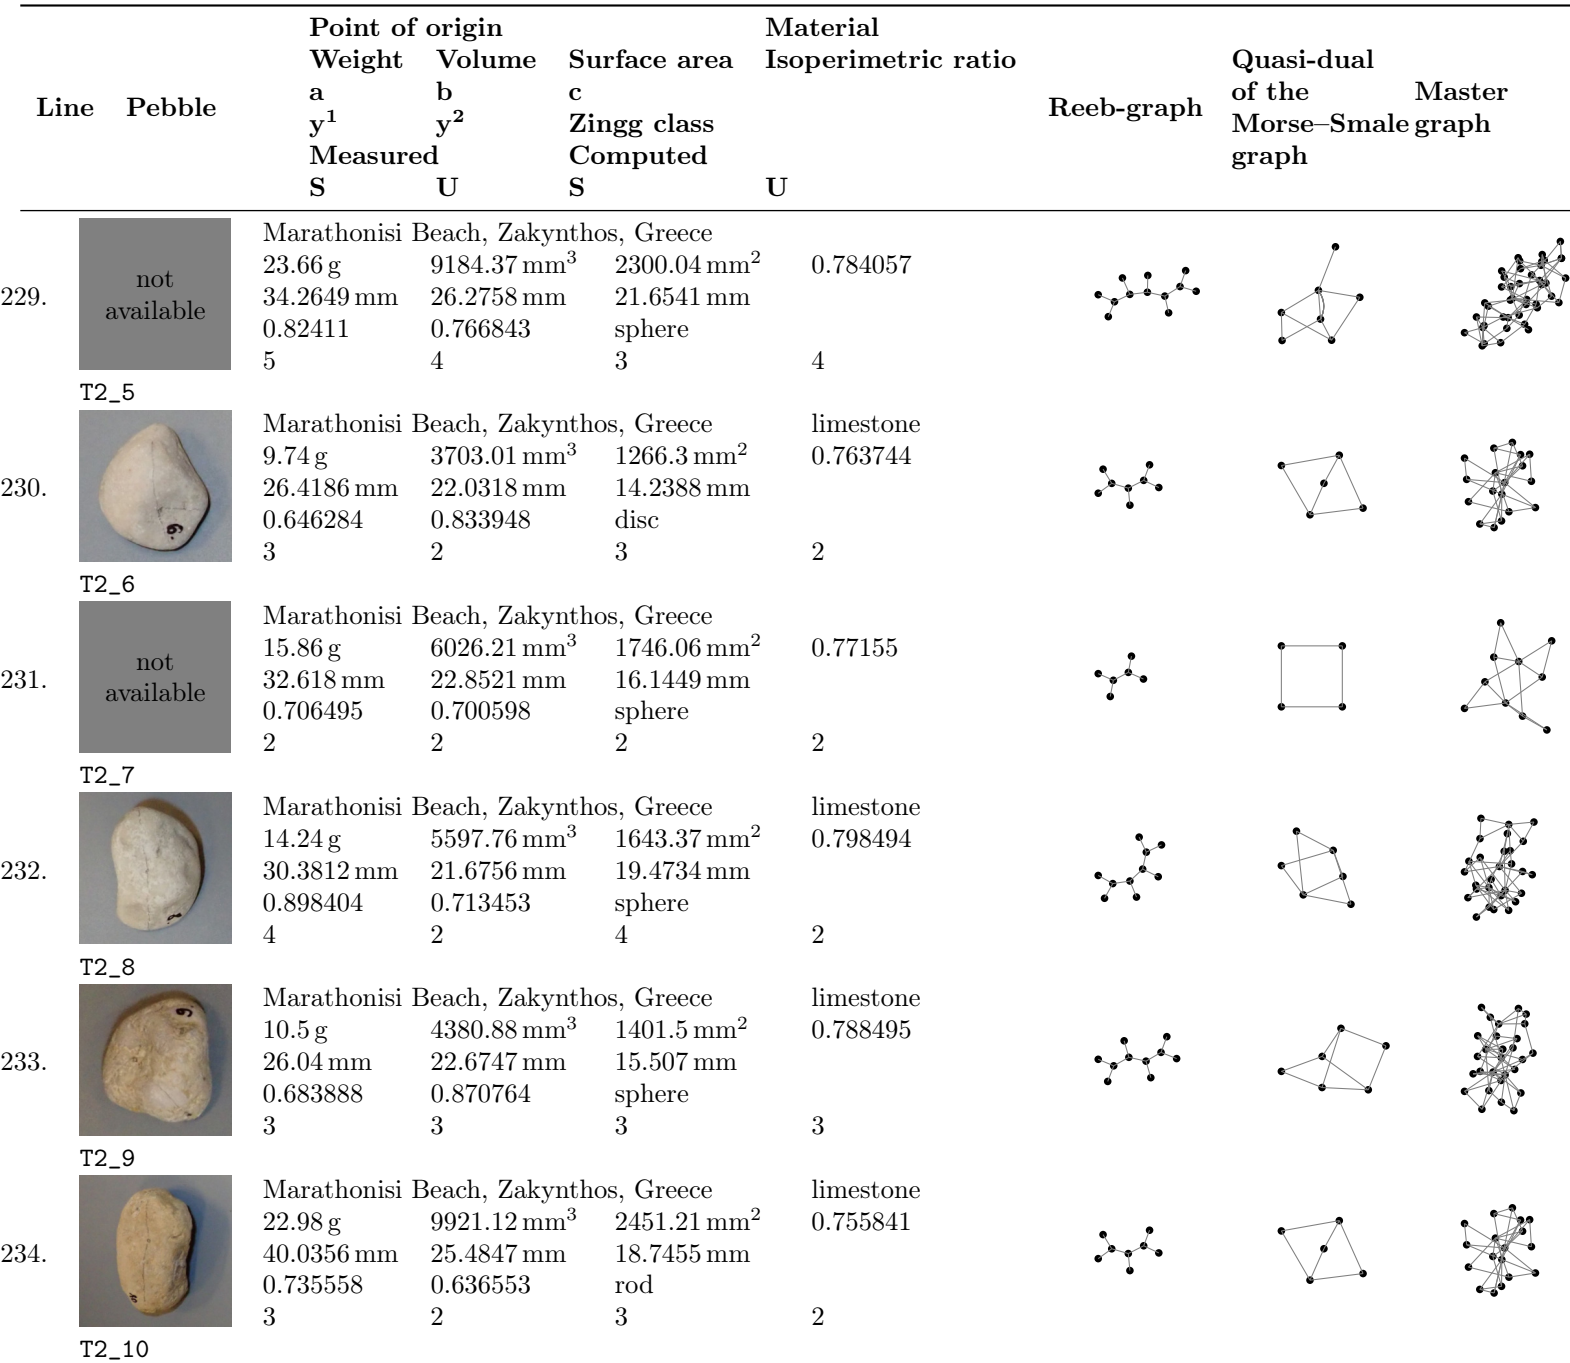 | 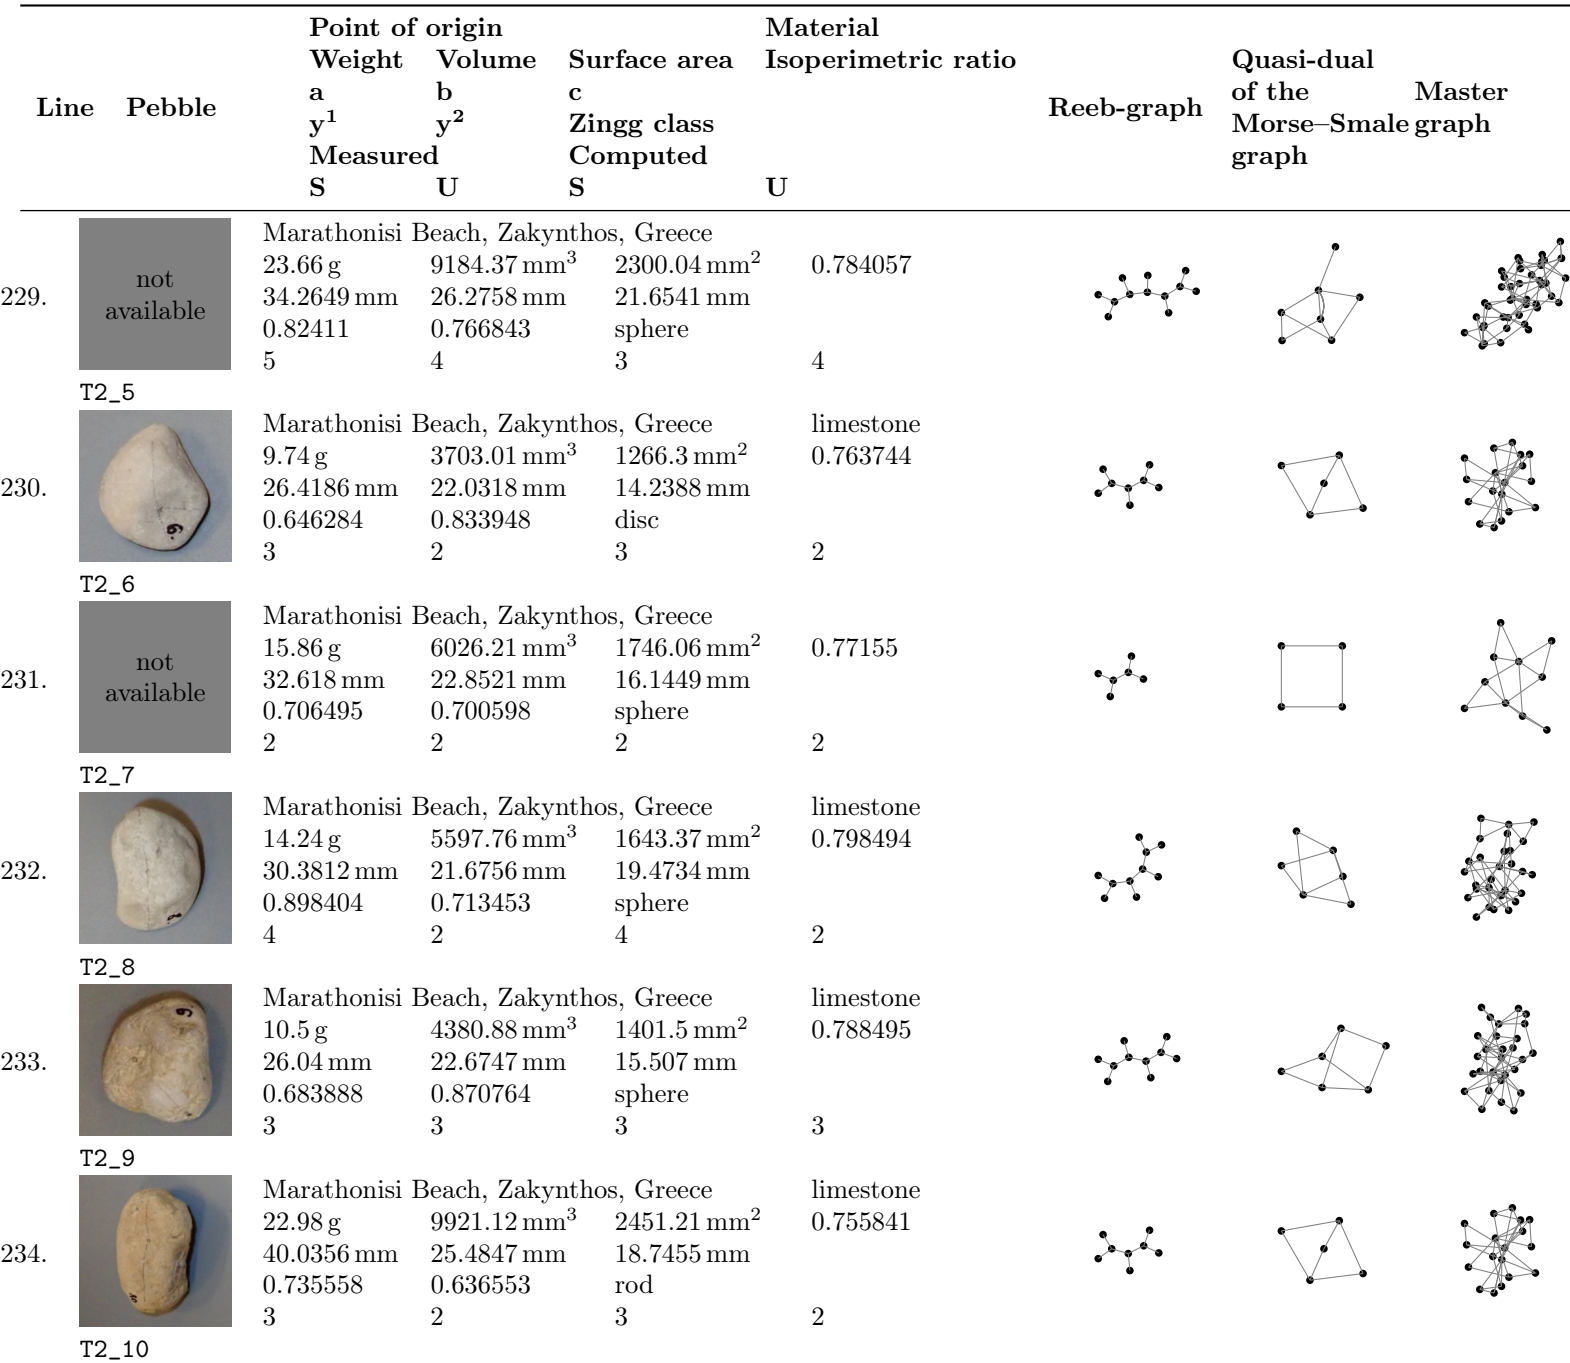 | 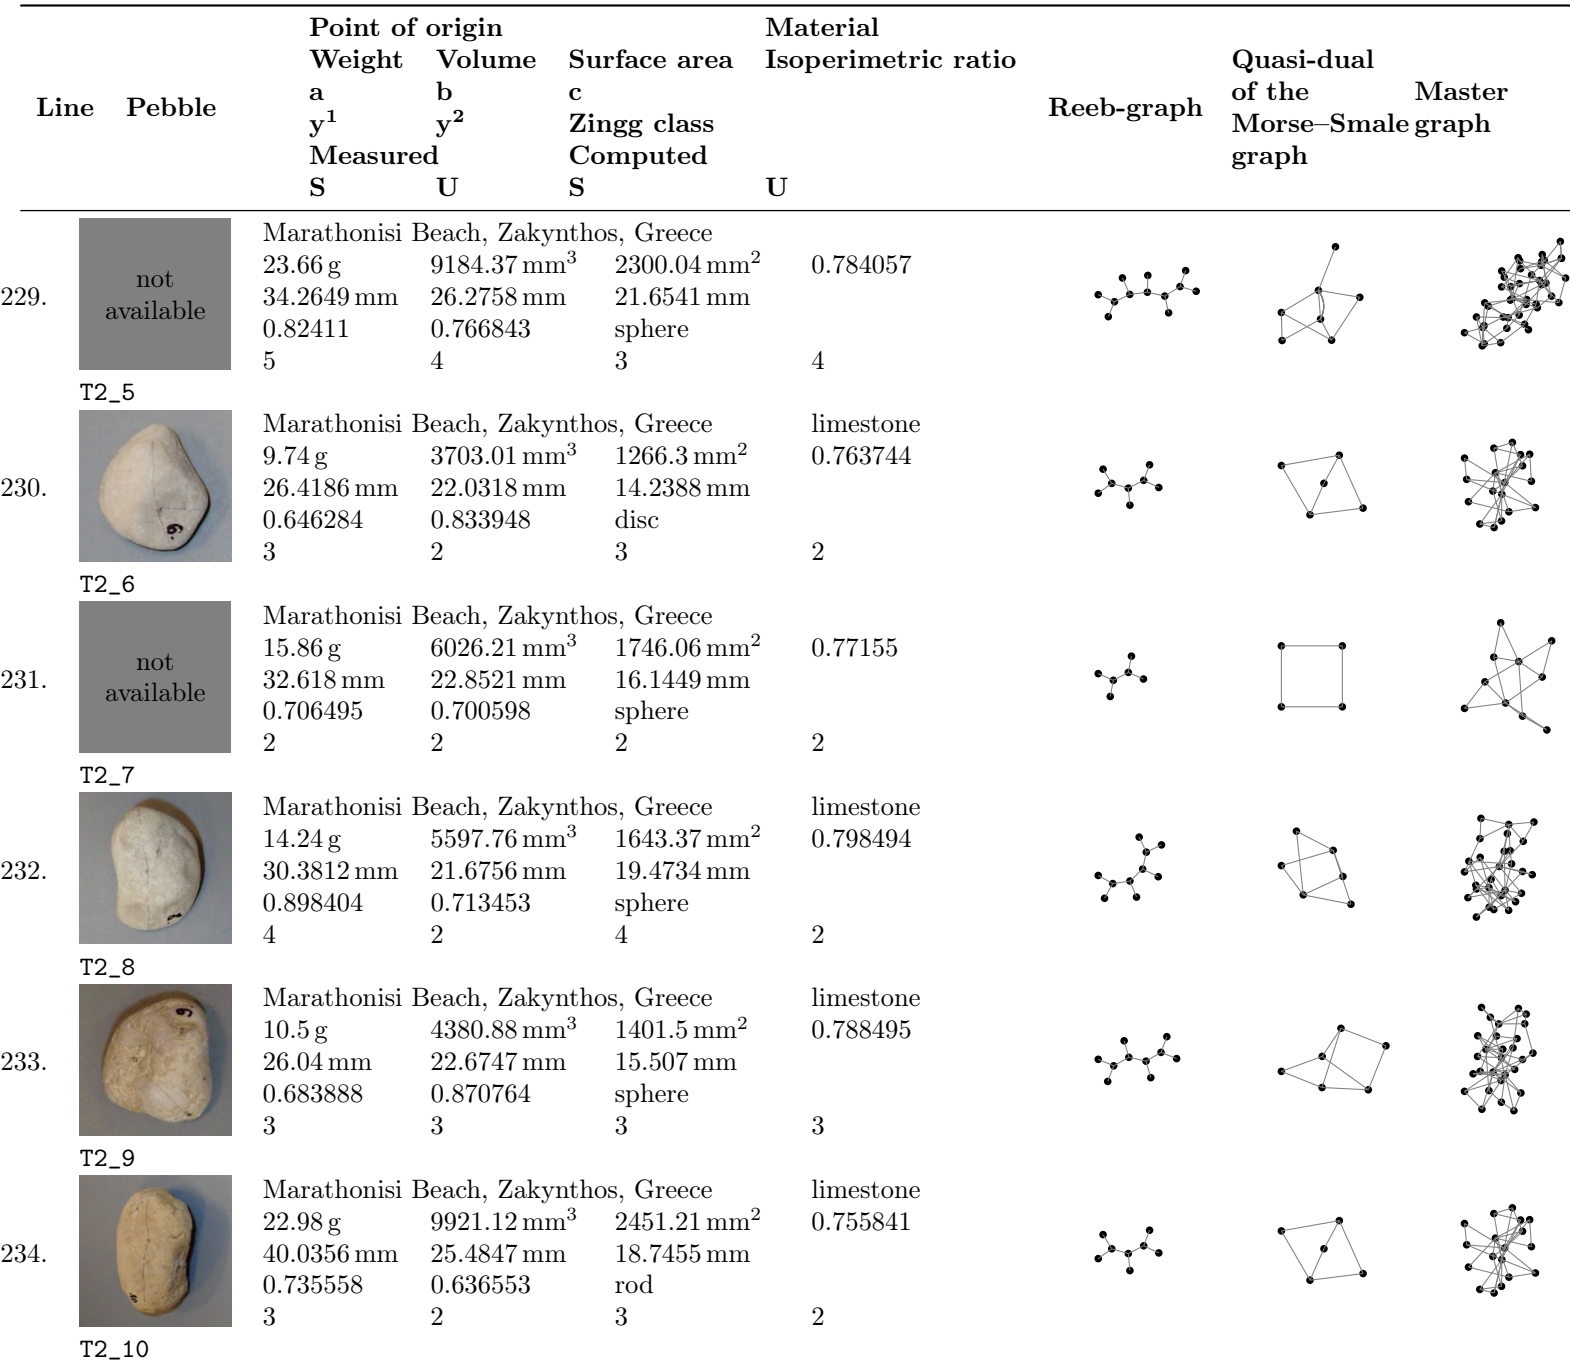 |
|      |                                                                                     | 22.98 g                              | 9921.12 mm <sup>3</sup> | 2451.21 mm <sup>2</sup>      |                       |                                                                                       |                                                                                       |                                                                                       |
|      |                                                                                     | 40.0356 mm                           | 25.4847 mm              | 18.7455 mm                   |                       |                                                                                       |                                                                                       |                                                                                       |
|      |                                                                                     | 0.735558                             | 0.636553                | rod                          |                       |                                                                                       |                                                                                       |                                                                                       |
|      |                                                                                     | 3                                    | 2                       | 3                            |                       |                                                                                       |                                                                                       |                                                                                       |
|      | T2_10                                                                               |                                      |                         |                              | 2                     |                                                                                       |                                                                                       |                                                                                       |

| Line | Pebble                                                                              | Point of origin                                                                |                                                                                     |                                                      | Material              | Reeb-graph                                                                            | Quasi-dual<br>of the<br>Morse–Smale<br>graph                                          | Master<br>graph                                                                       |
|------|-------------------------------------------------------------------------------------|--------------------------------------------------------------------------------|-------------------------------------------------------------------------------------|------------------------------------------------------|-----------------------|---------------------------------------------------------------------------------------|---------------------------------------------------------------------------------------|---------------------------------------------------------------------------------------|
|      |                                                                                     | Weight                                                                         | Volume                                                                              | Surface area                                         |                       |                                                                                       |                                                                                       |                                                                                       |
|      |                                                                                     | a                                                                              | b                                                                                   | c                                                    |                       |                                                                                       |                                                                                       |                                                                                       |
|      |                                                                                     | y <sup>1</sup><br>Measured<br>S                                                | y <sup>2</sup><br>U                                                                 | Zingg class<br>Computed<br>S                         |                       |                                                                                       |                                                                                       |                                                                                       |
| 235. | 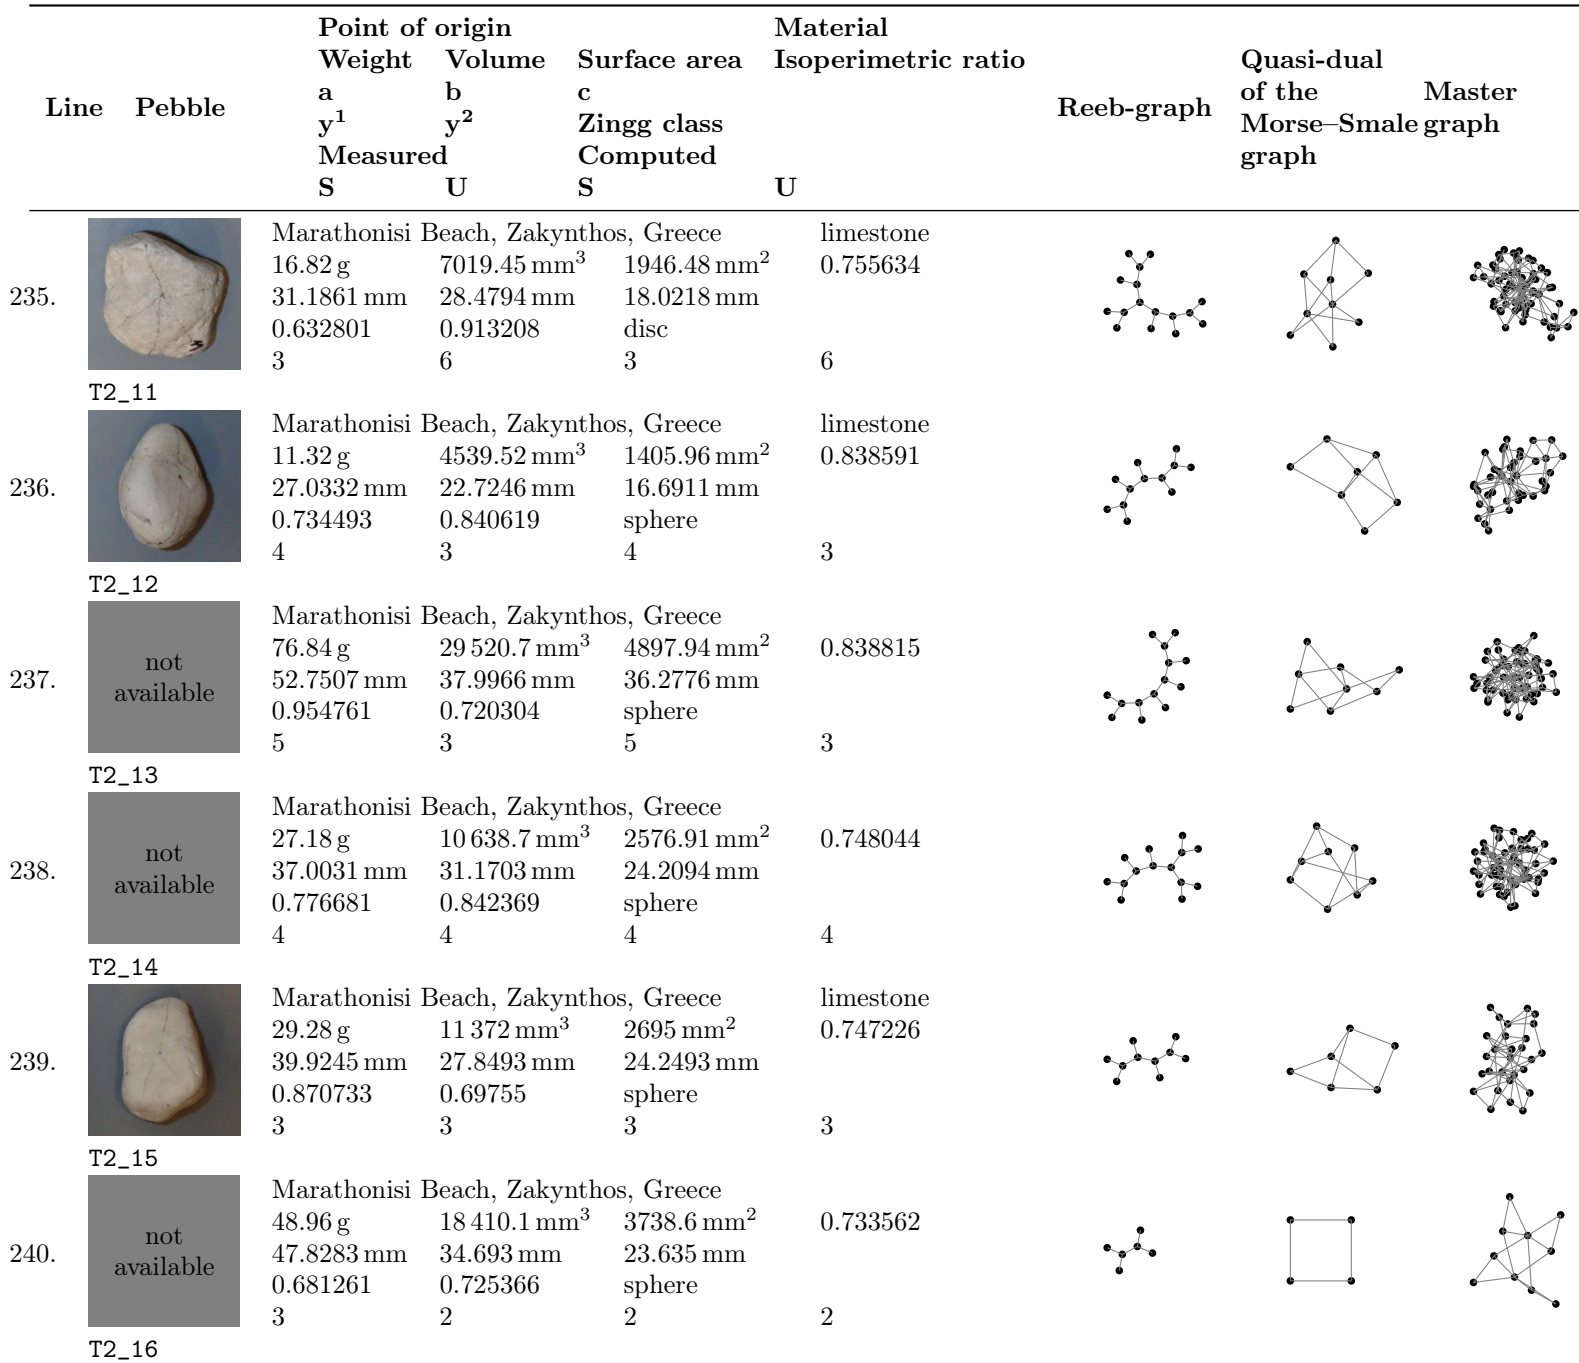   | Marathonisi Beach, Zakynthos, Greece<br>16.82 g<br>31.1861 mm<br>0.632801<br>3 | Beach, Zakynthos, Greece<br>7019.45 mm <sup>3</sup><br>28.4794 mm<br>0.913208<br>6  | 1946.48 mm <sup>2</sup><br>18.0218 mm<br>disc<br>3   | limestone<br>0.755634 | 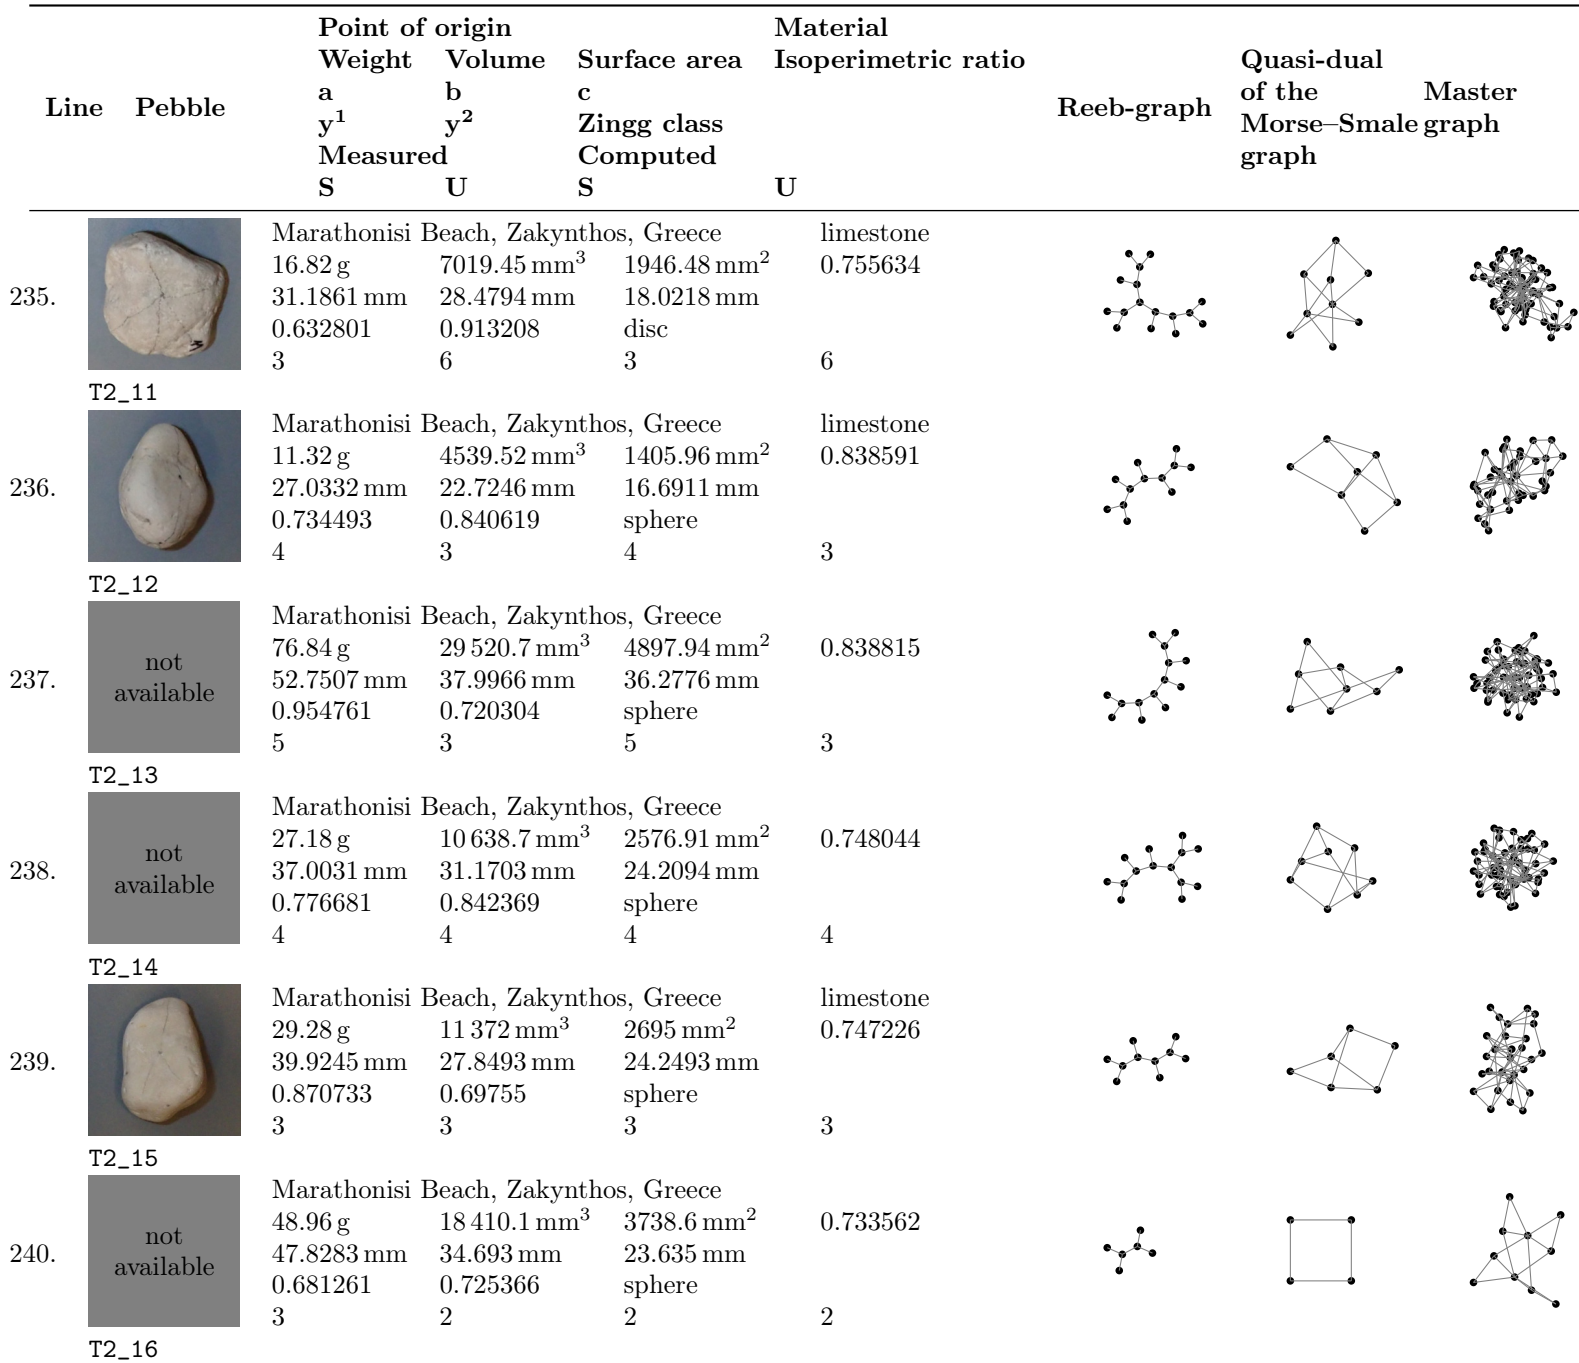   | 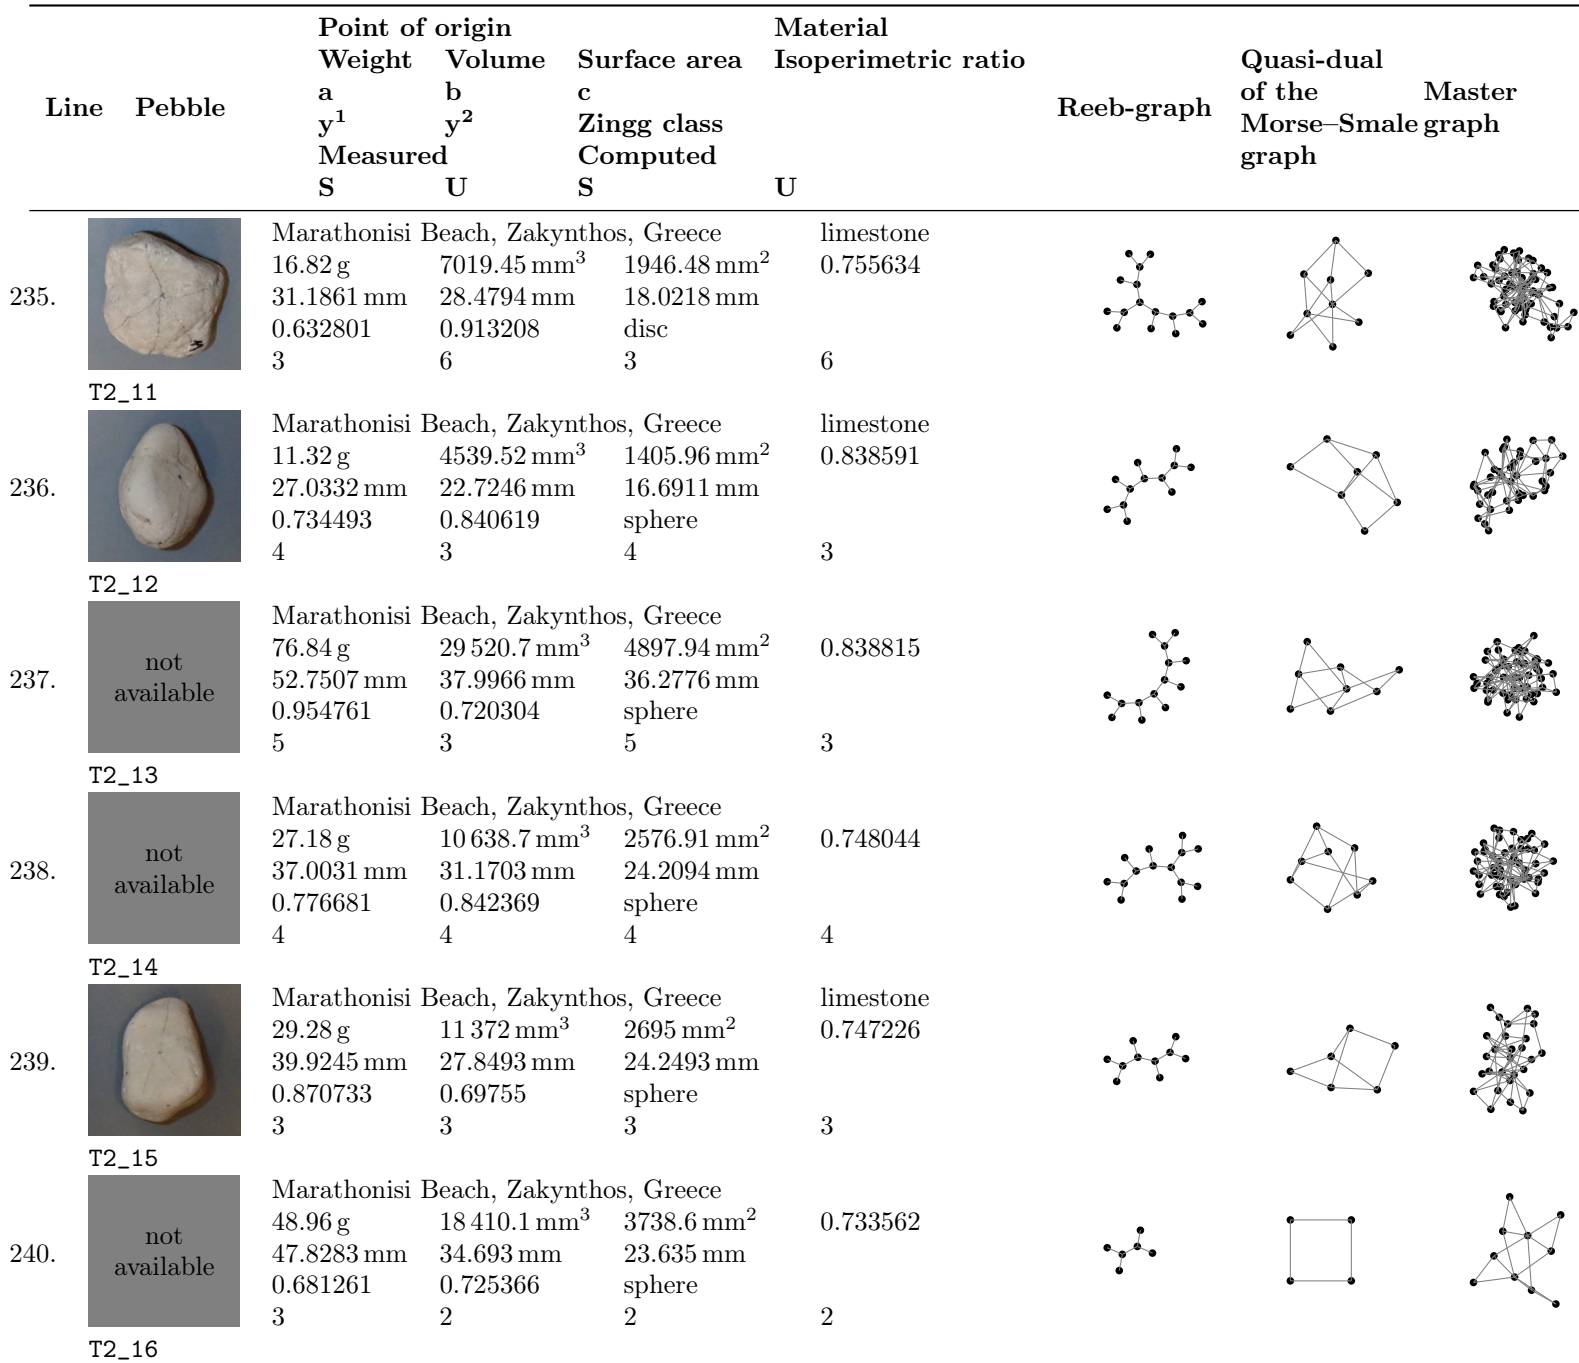   | 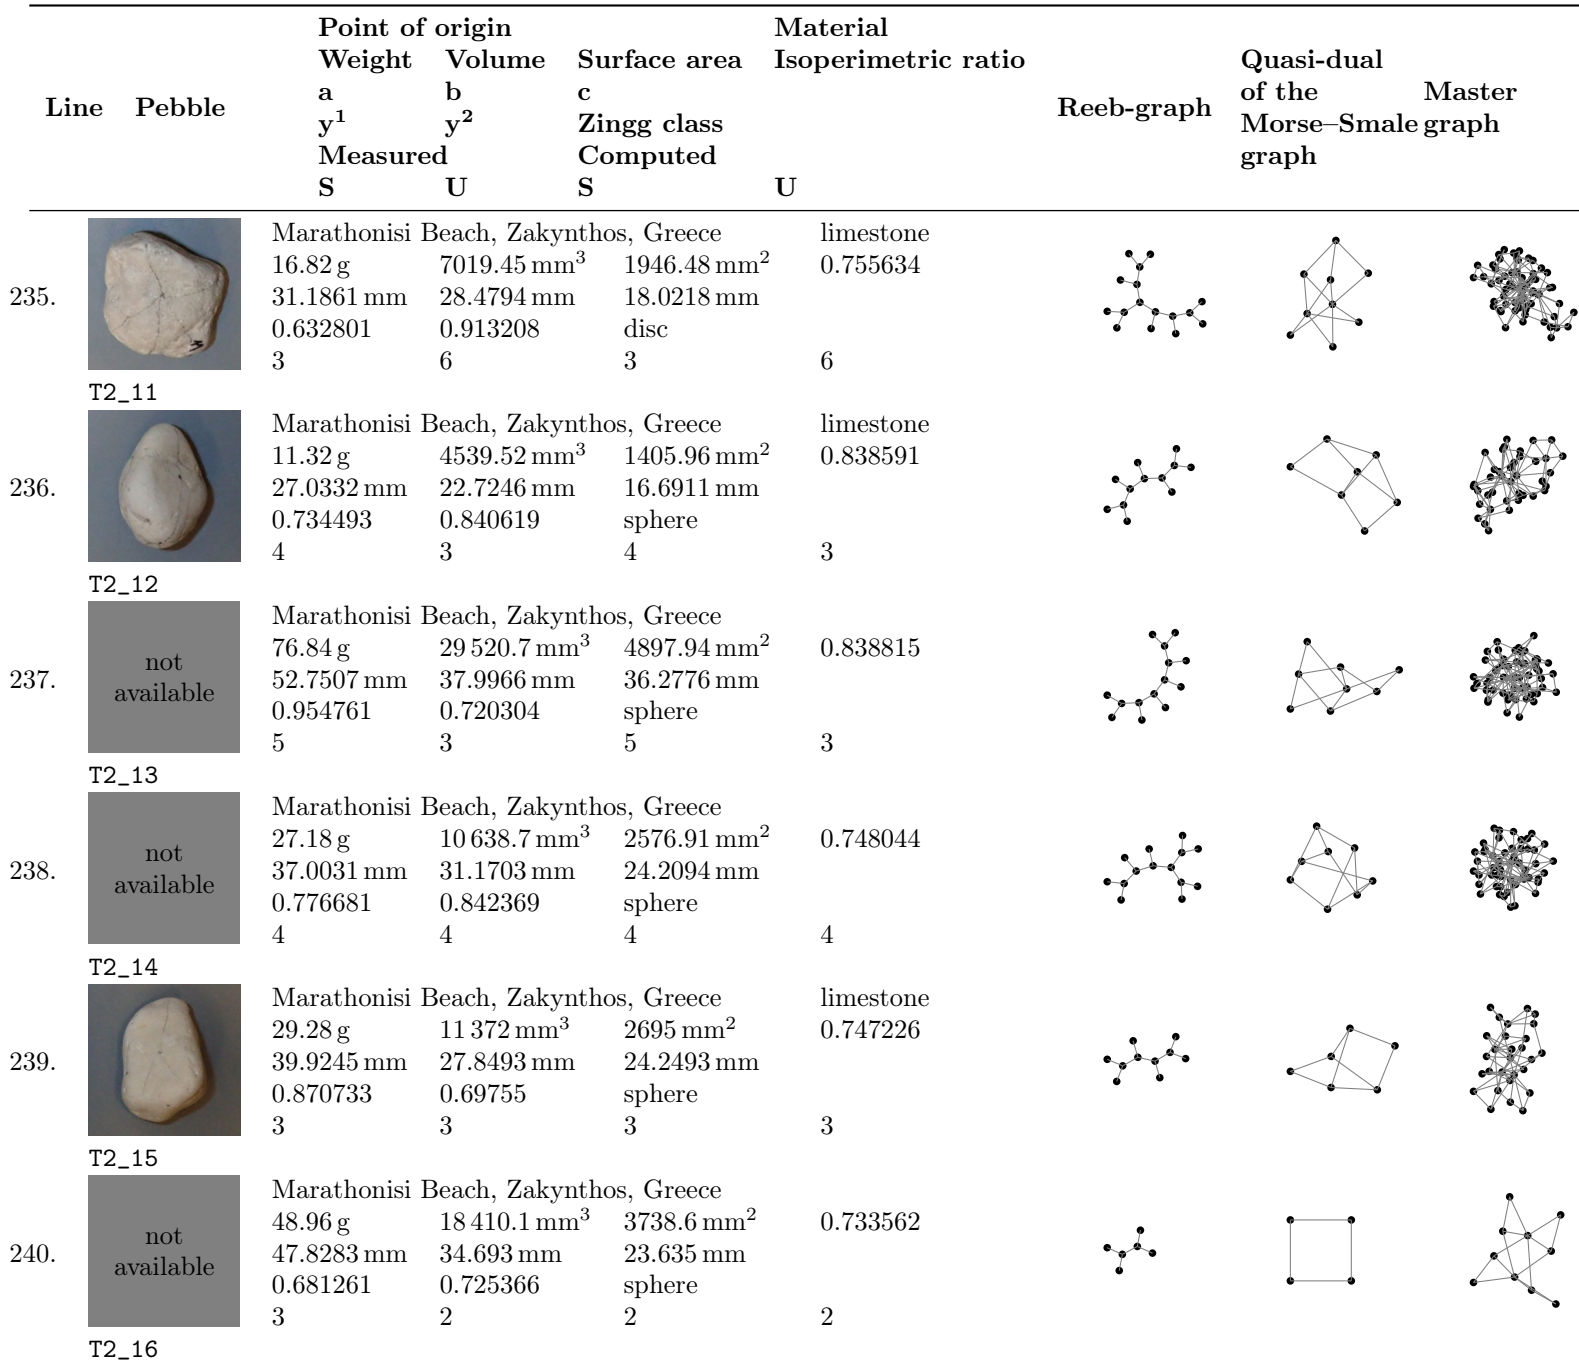   |
|      | T2_11                                                                               |                                                                                |                                                                                     |                                                      |                       |                                                                                       |                                                                                       |                                                                                       |
| 236. | 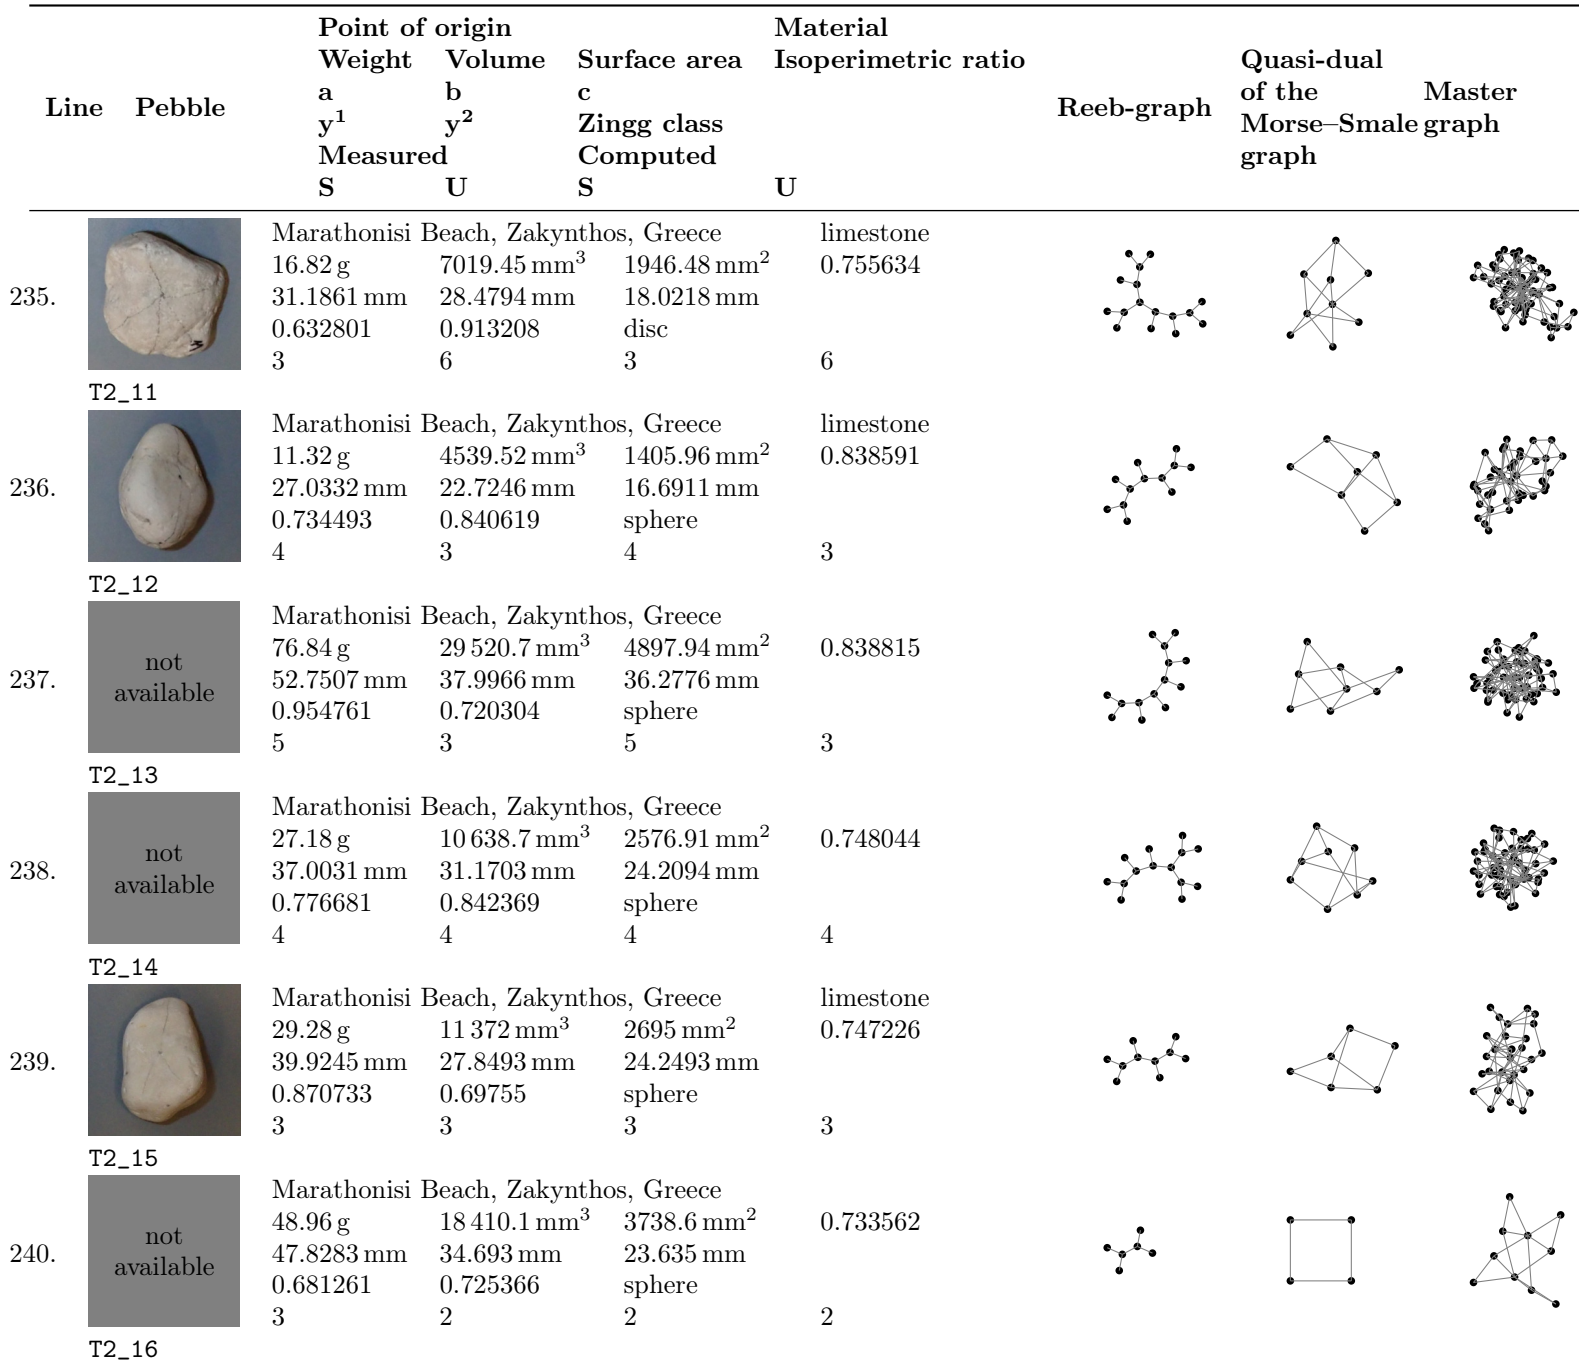   | Marathonisi Beach, Zakynthos, Greece<br>11.32 g<br>27.0332 mm<br>0.734493<br>4 | Beach, Zakynthos, Greece<br>4539.52 mm <sup>3</sup><br>22.7246 mm<br>0.840619<br>3  | 1405.96 mm <sup>2</sup><br>16.6911 mm<br>sphere<br>4 | limestone<br>0.838591 | 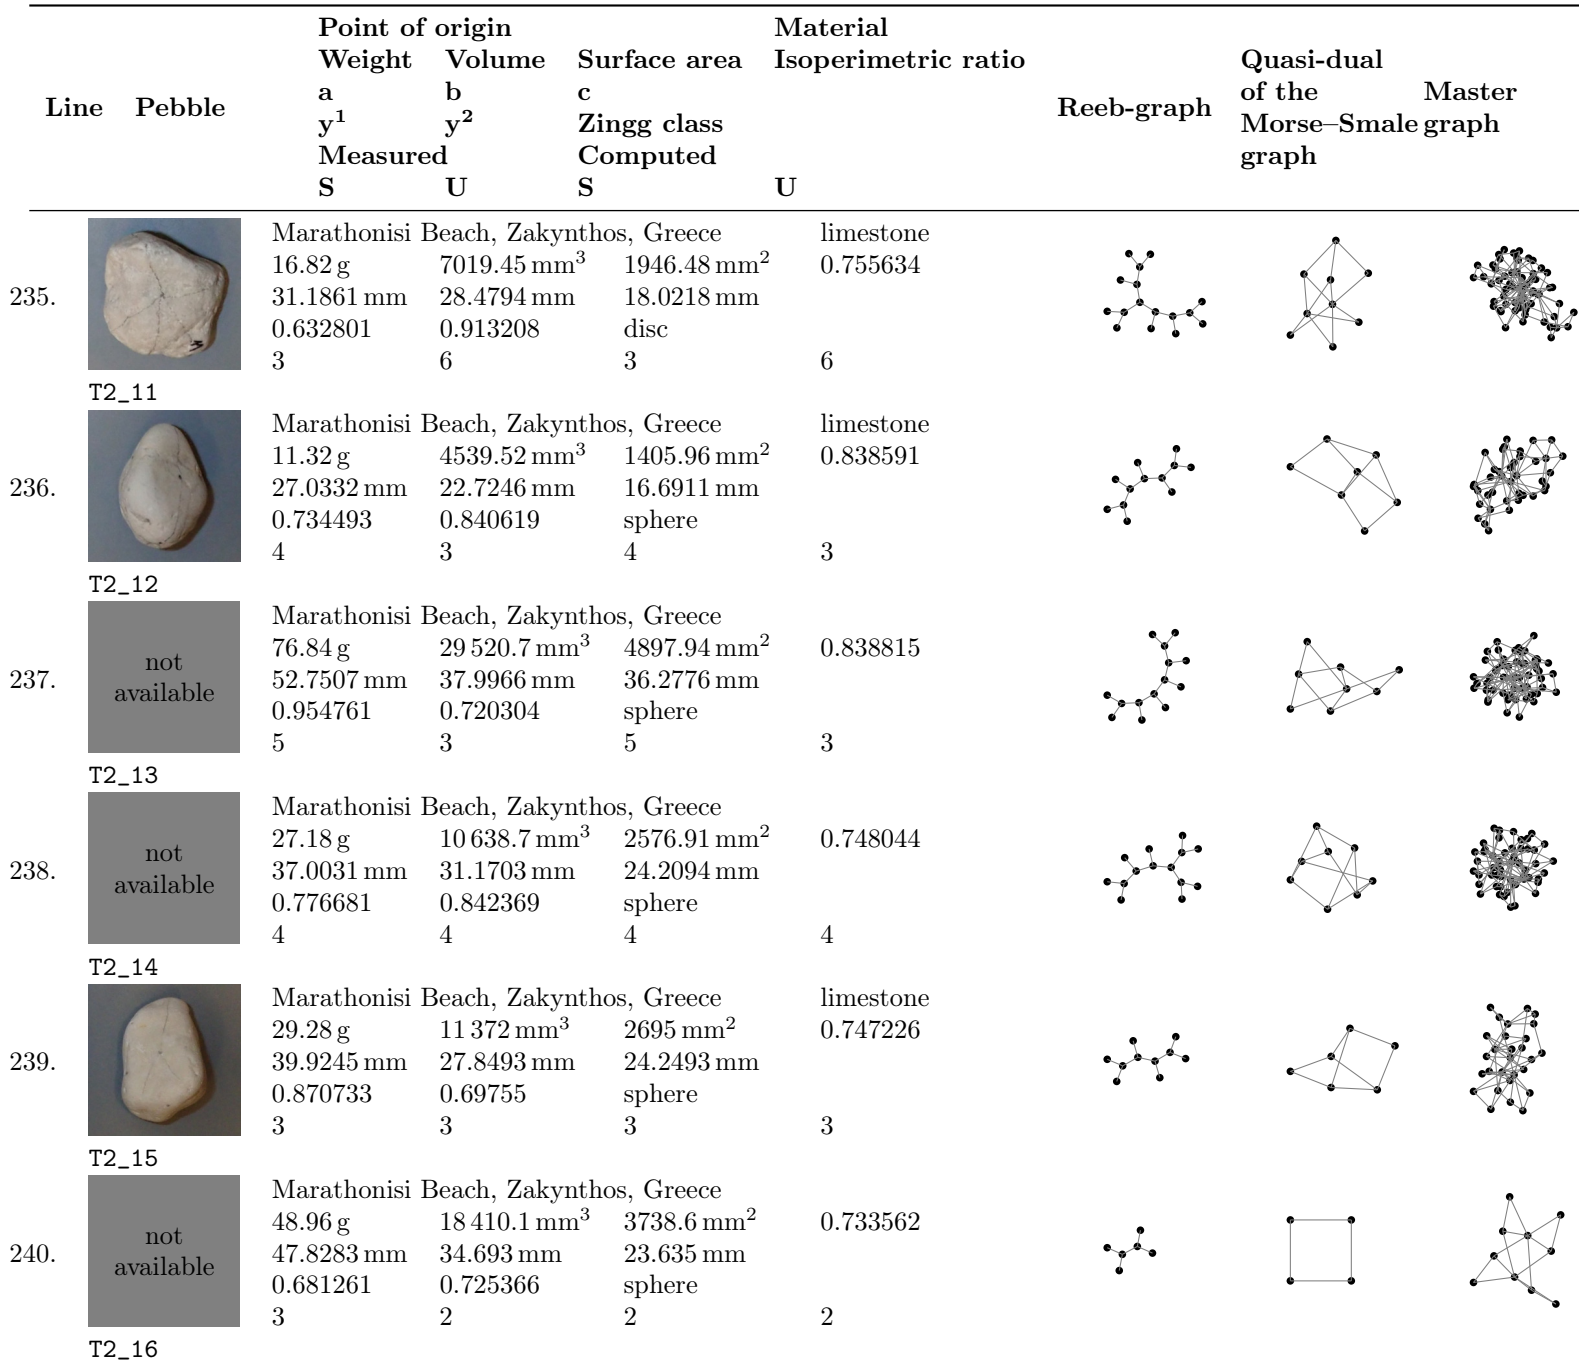   | 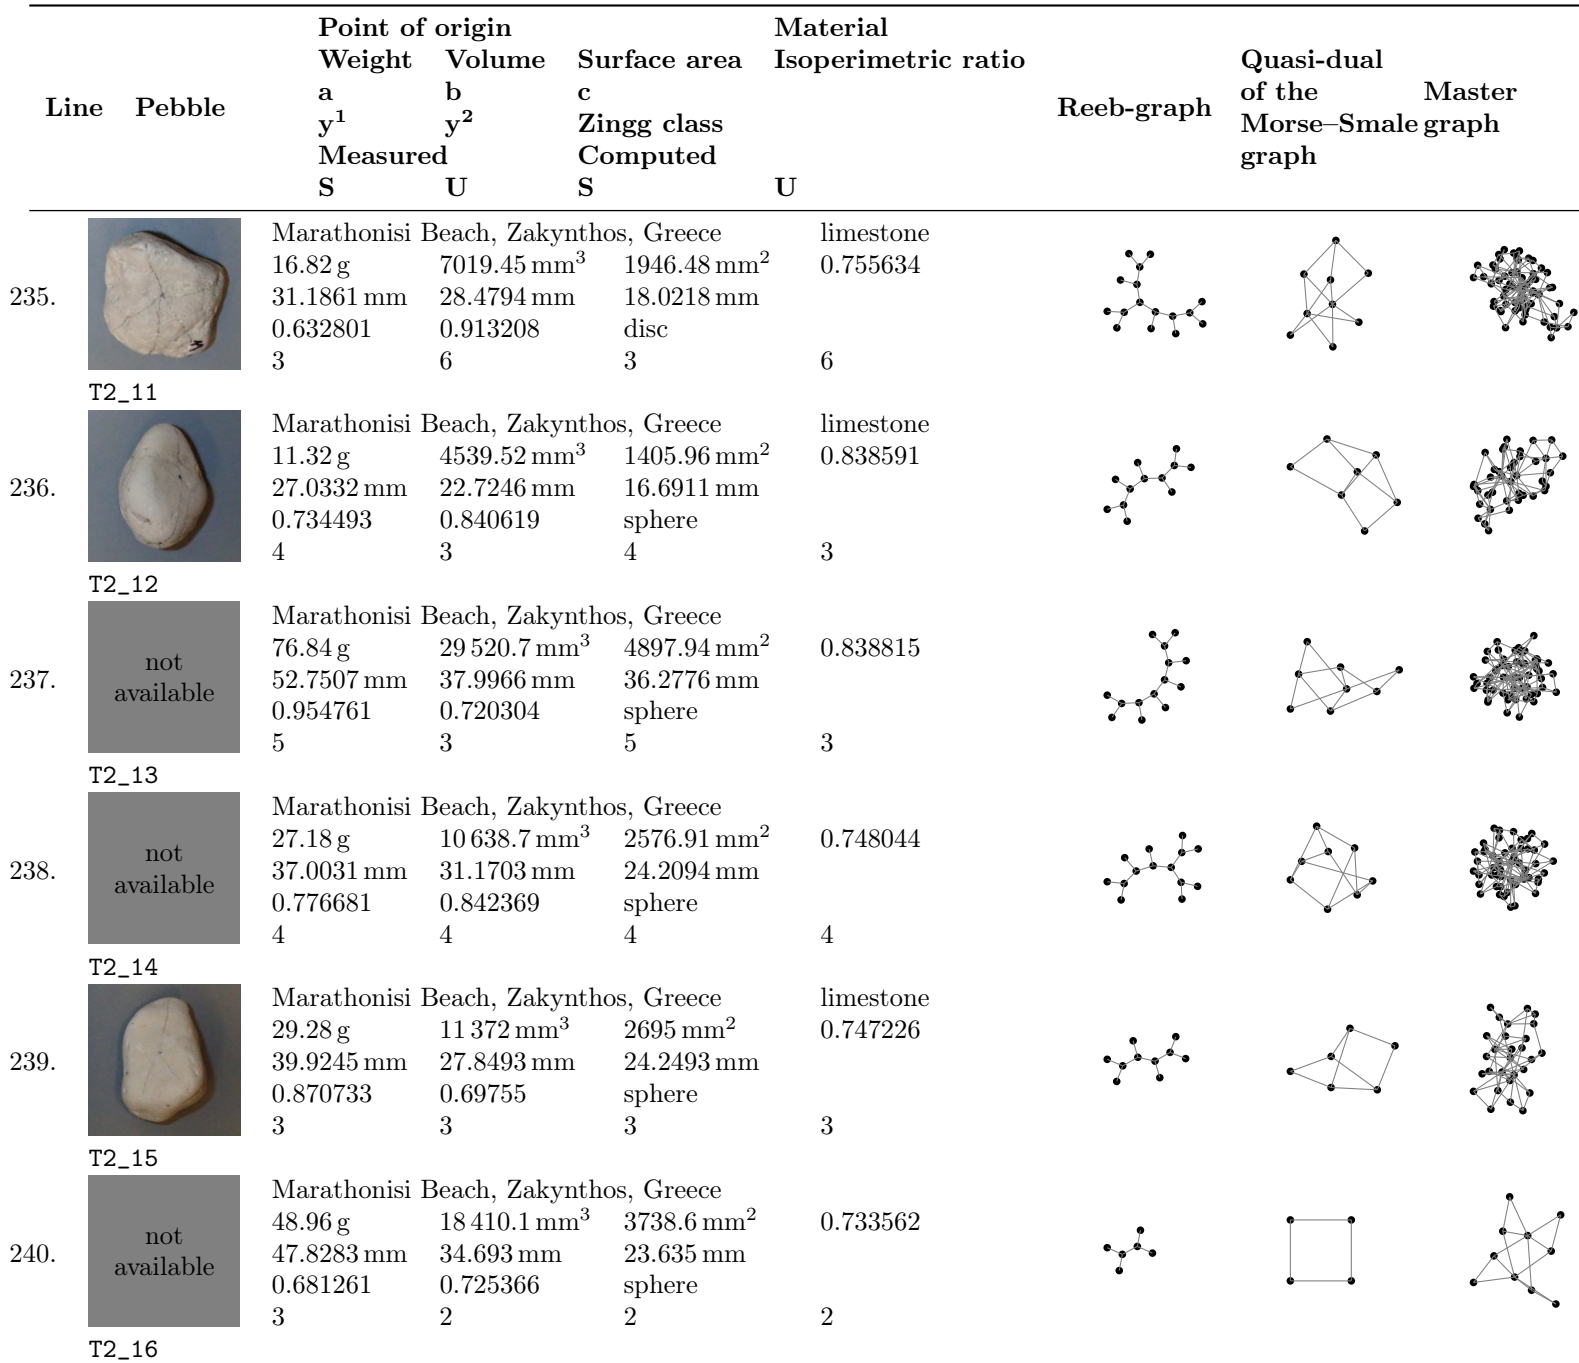   | 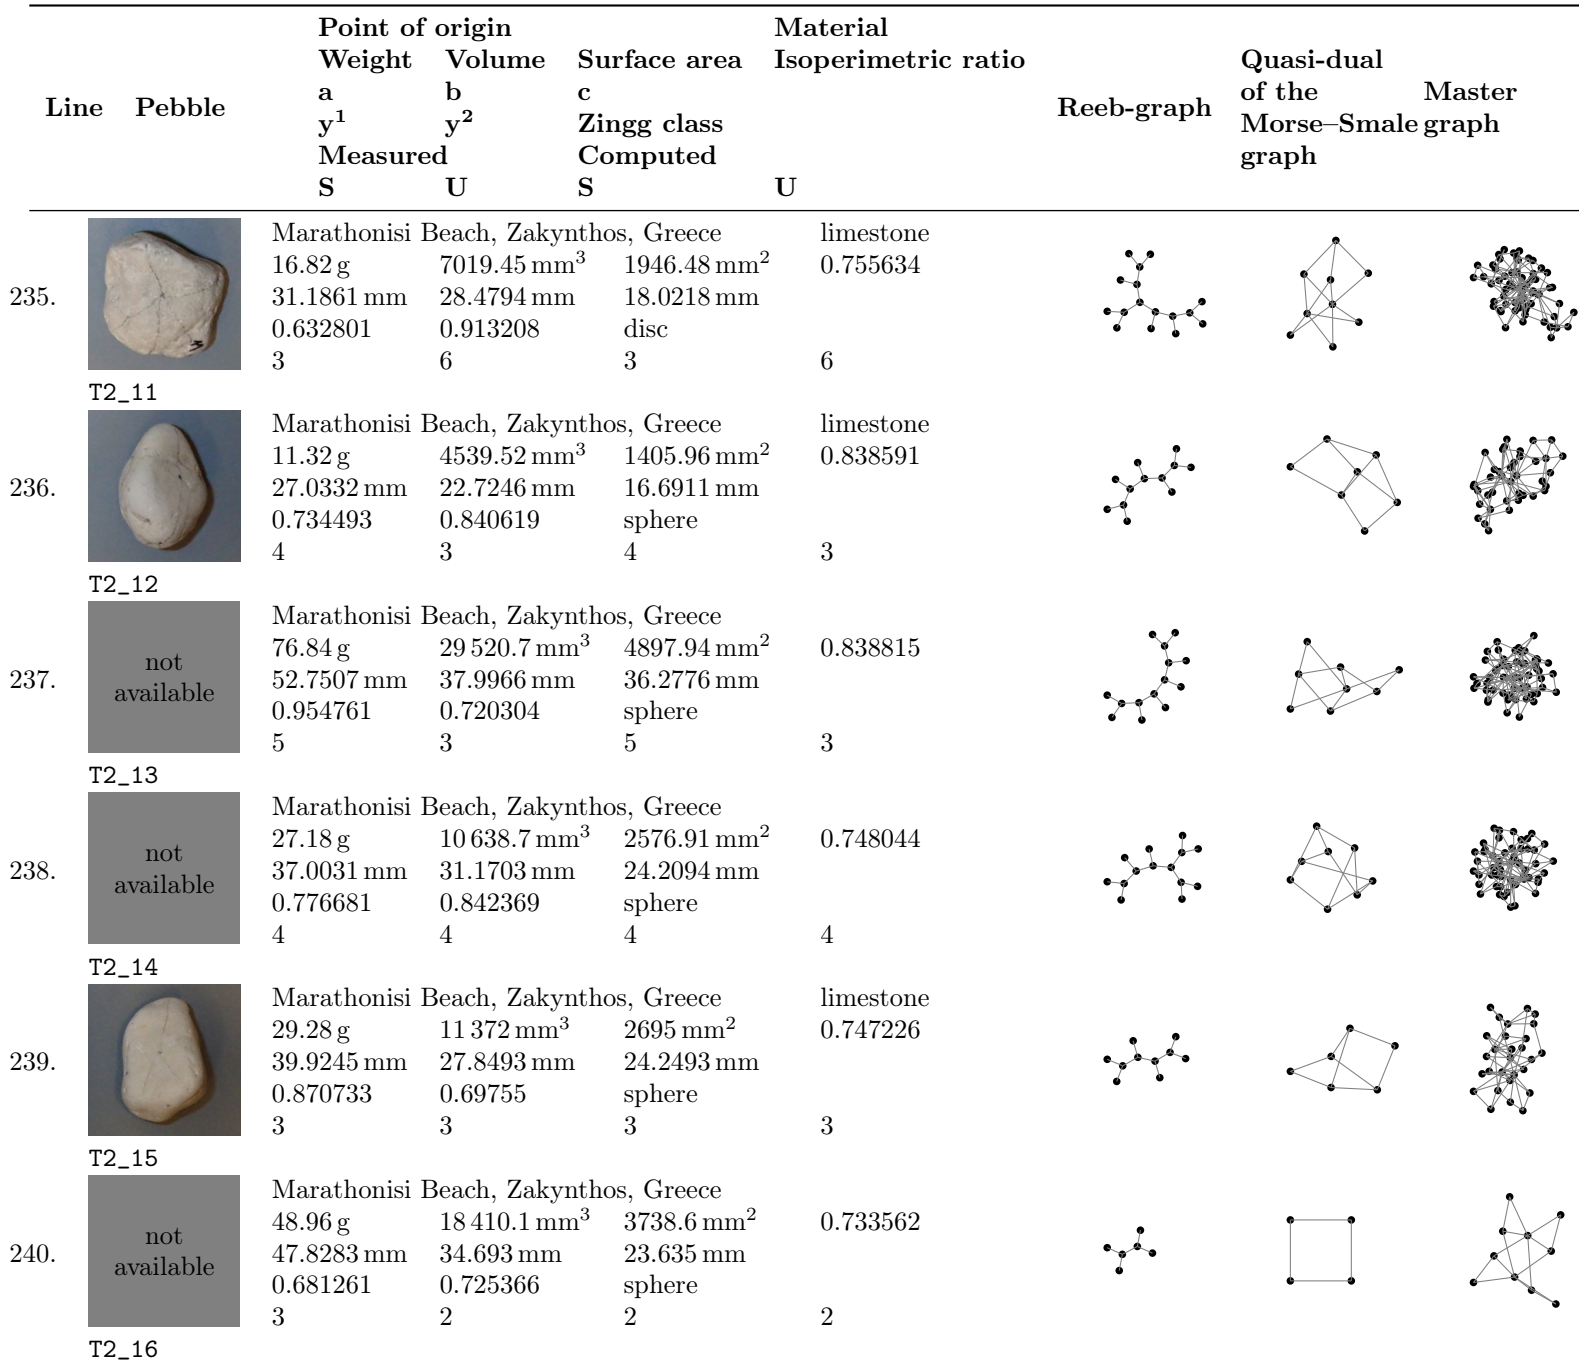   |
|      | T2_12                                                                               |                                                                                |                                                                                     |                                                      |                       |                                                                                       |                                                                                       |                                                                                       |
| 237. | 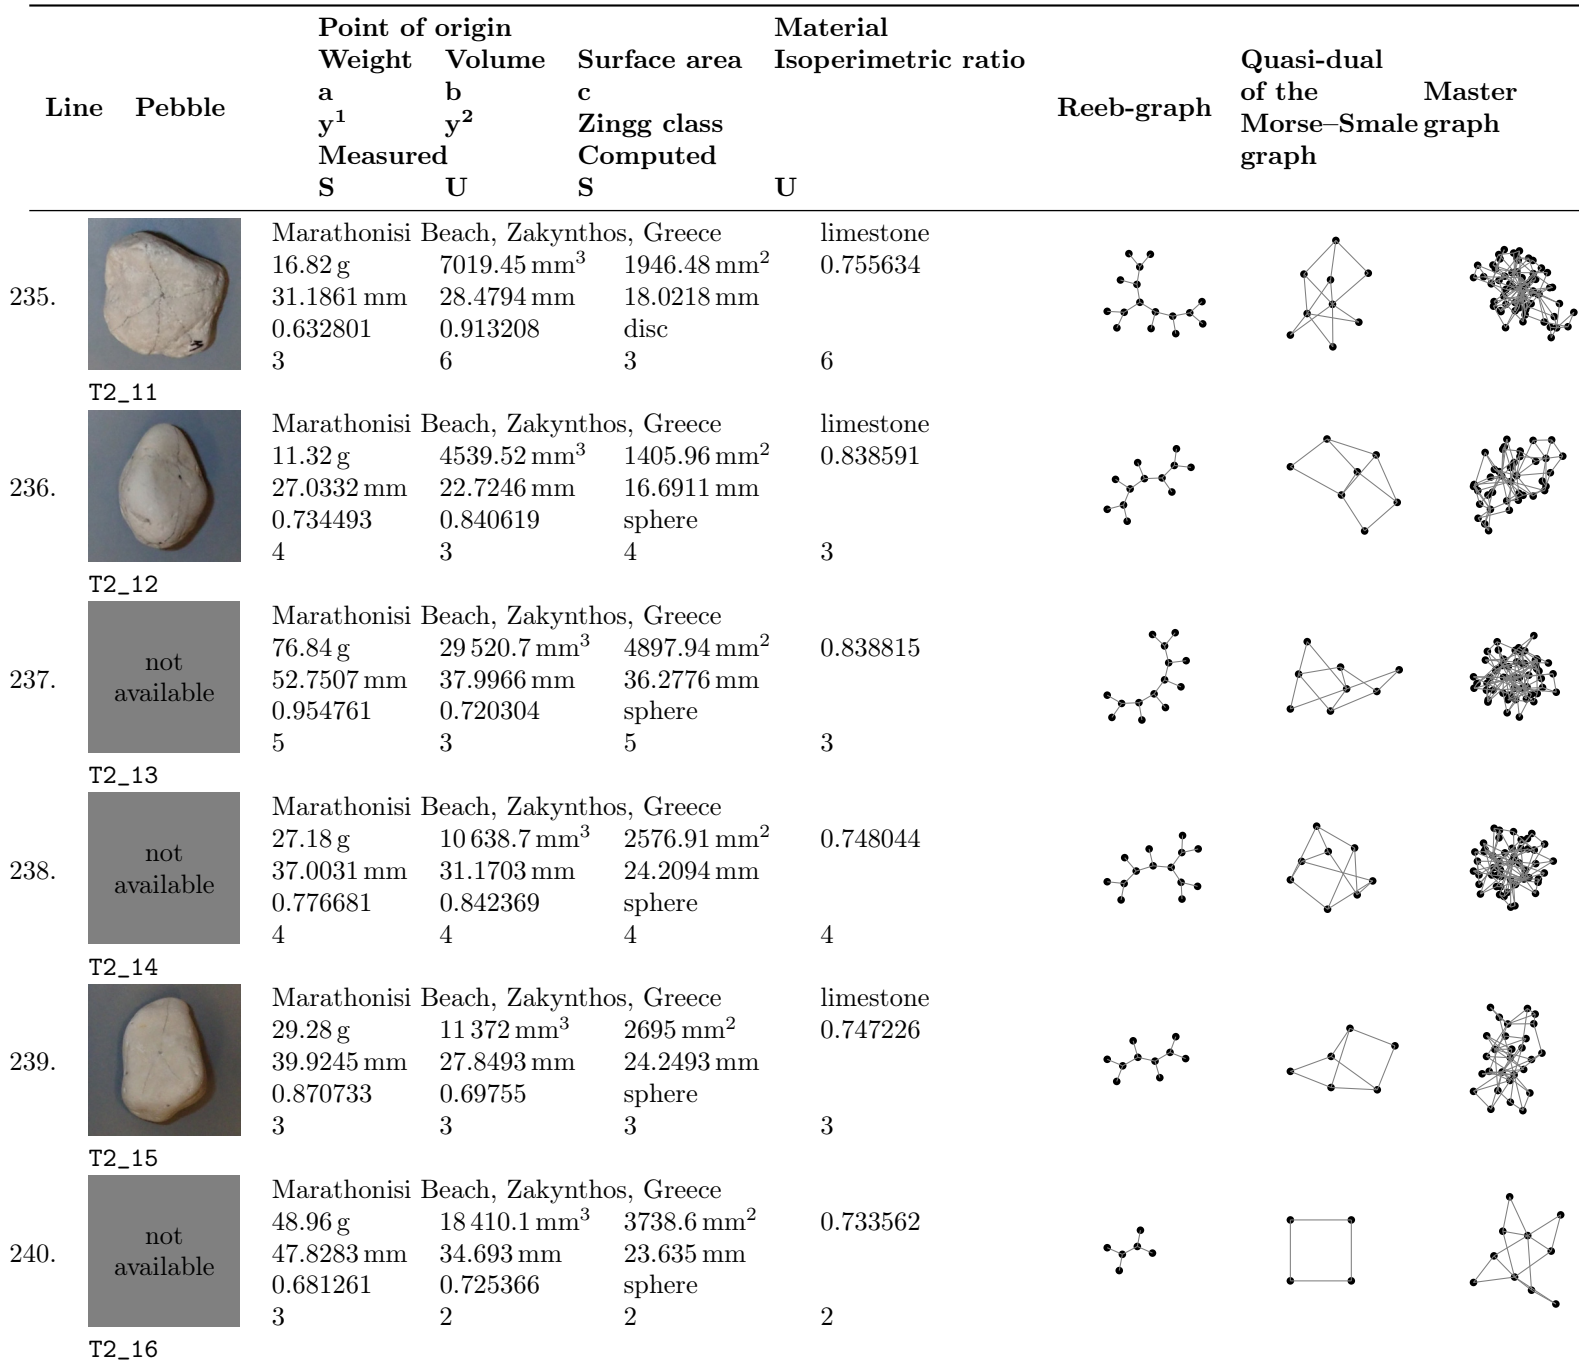   | Marathonisi Beach, Zakynthos, Greece<br>76.84 g<br>52.7507 mm<br>0.954761<br>5 | Beach, Zakynthos, Greece<br>29 520.7 mm <sup>3</sup><br>37.9966 mm<br>0.720304<br>3 | 4897.94 mm <sup>2</sup><br>36.2776 mm<br>sphere<br>5 | 0.838815              | 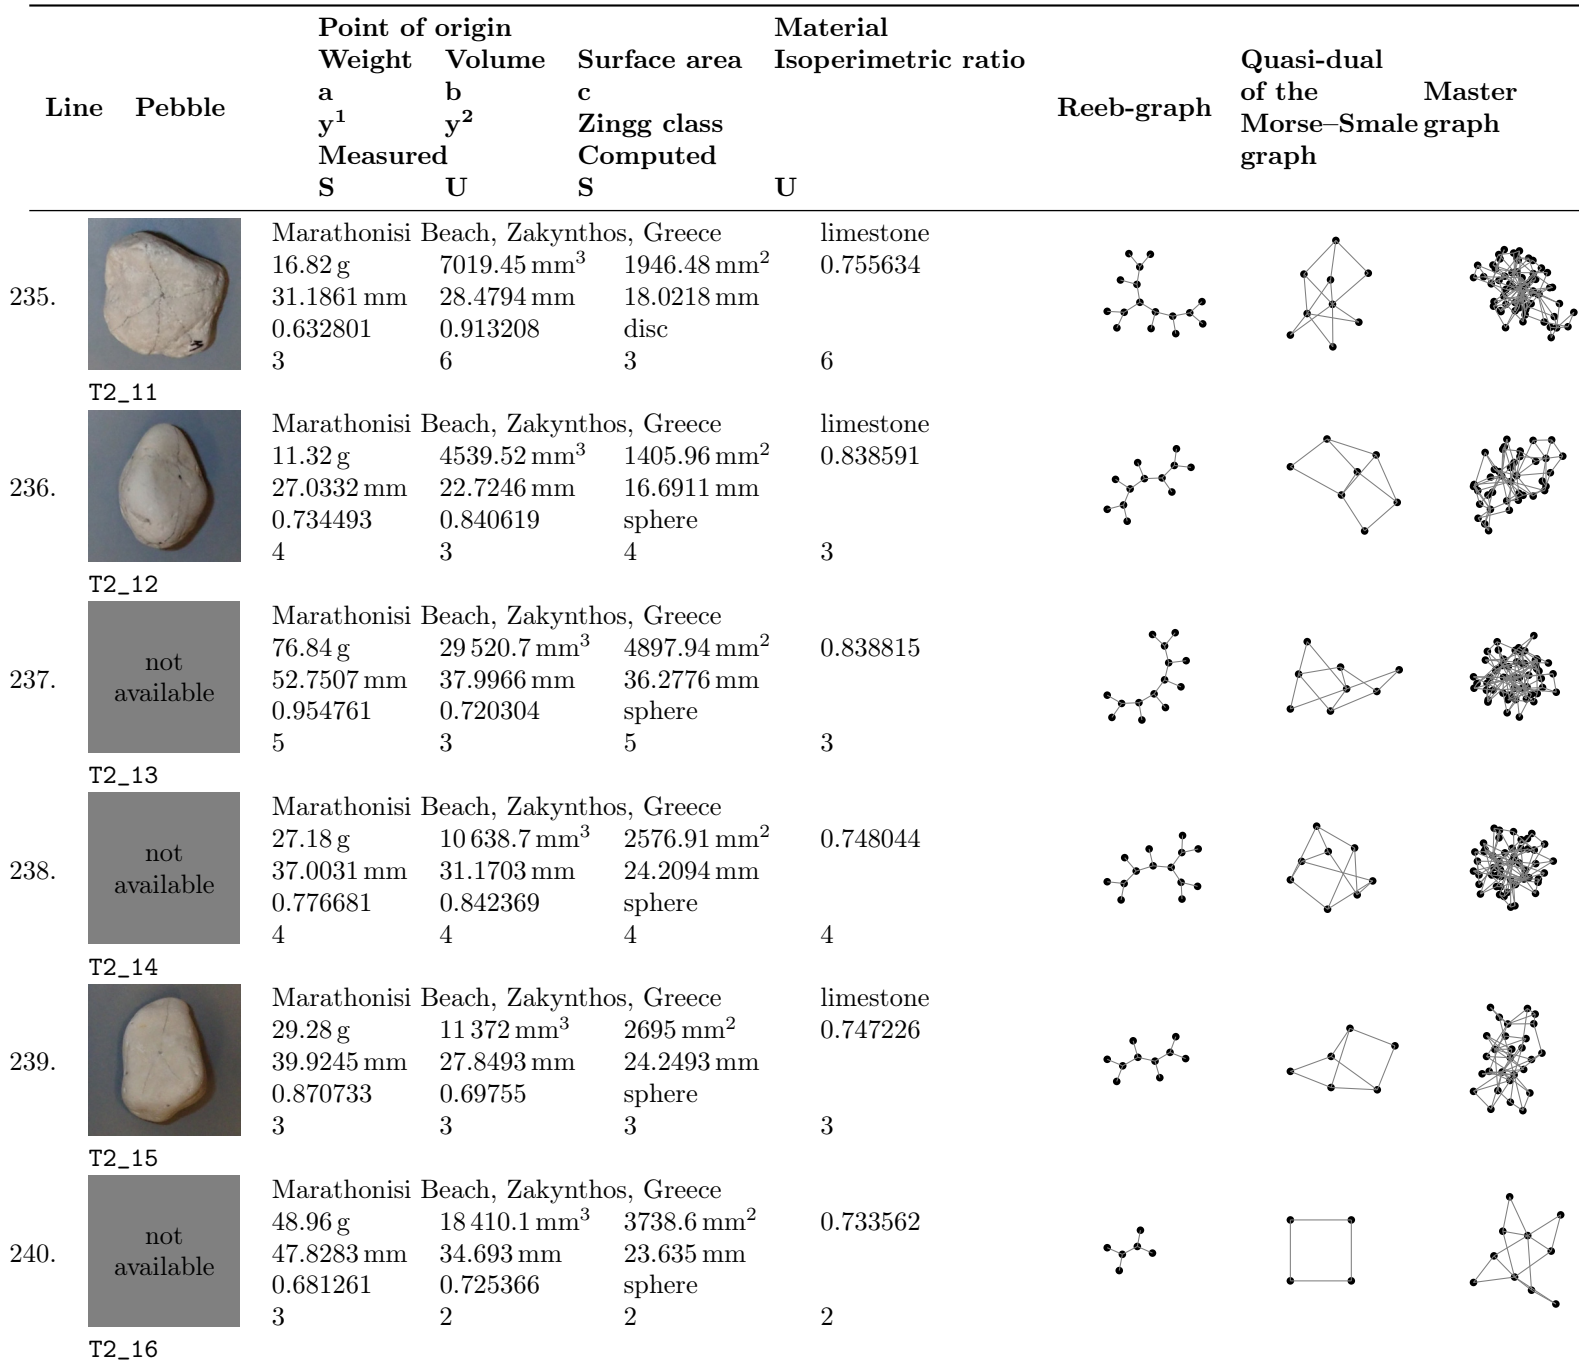   | 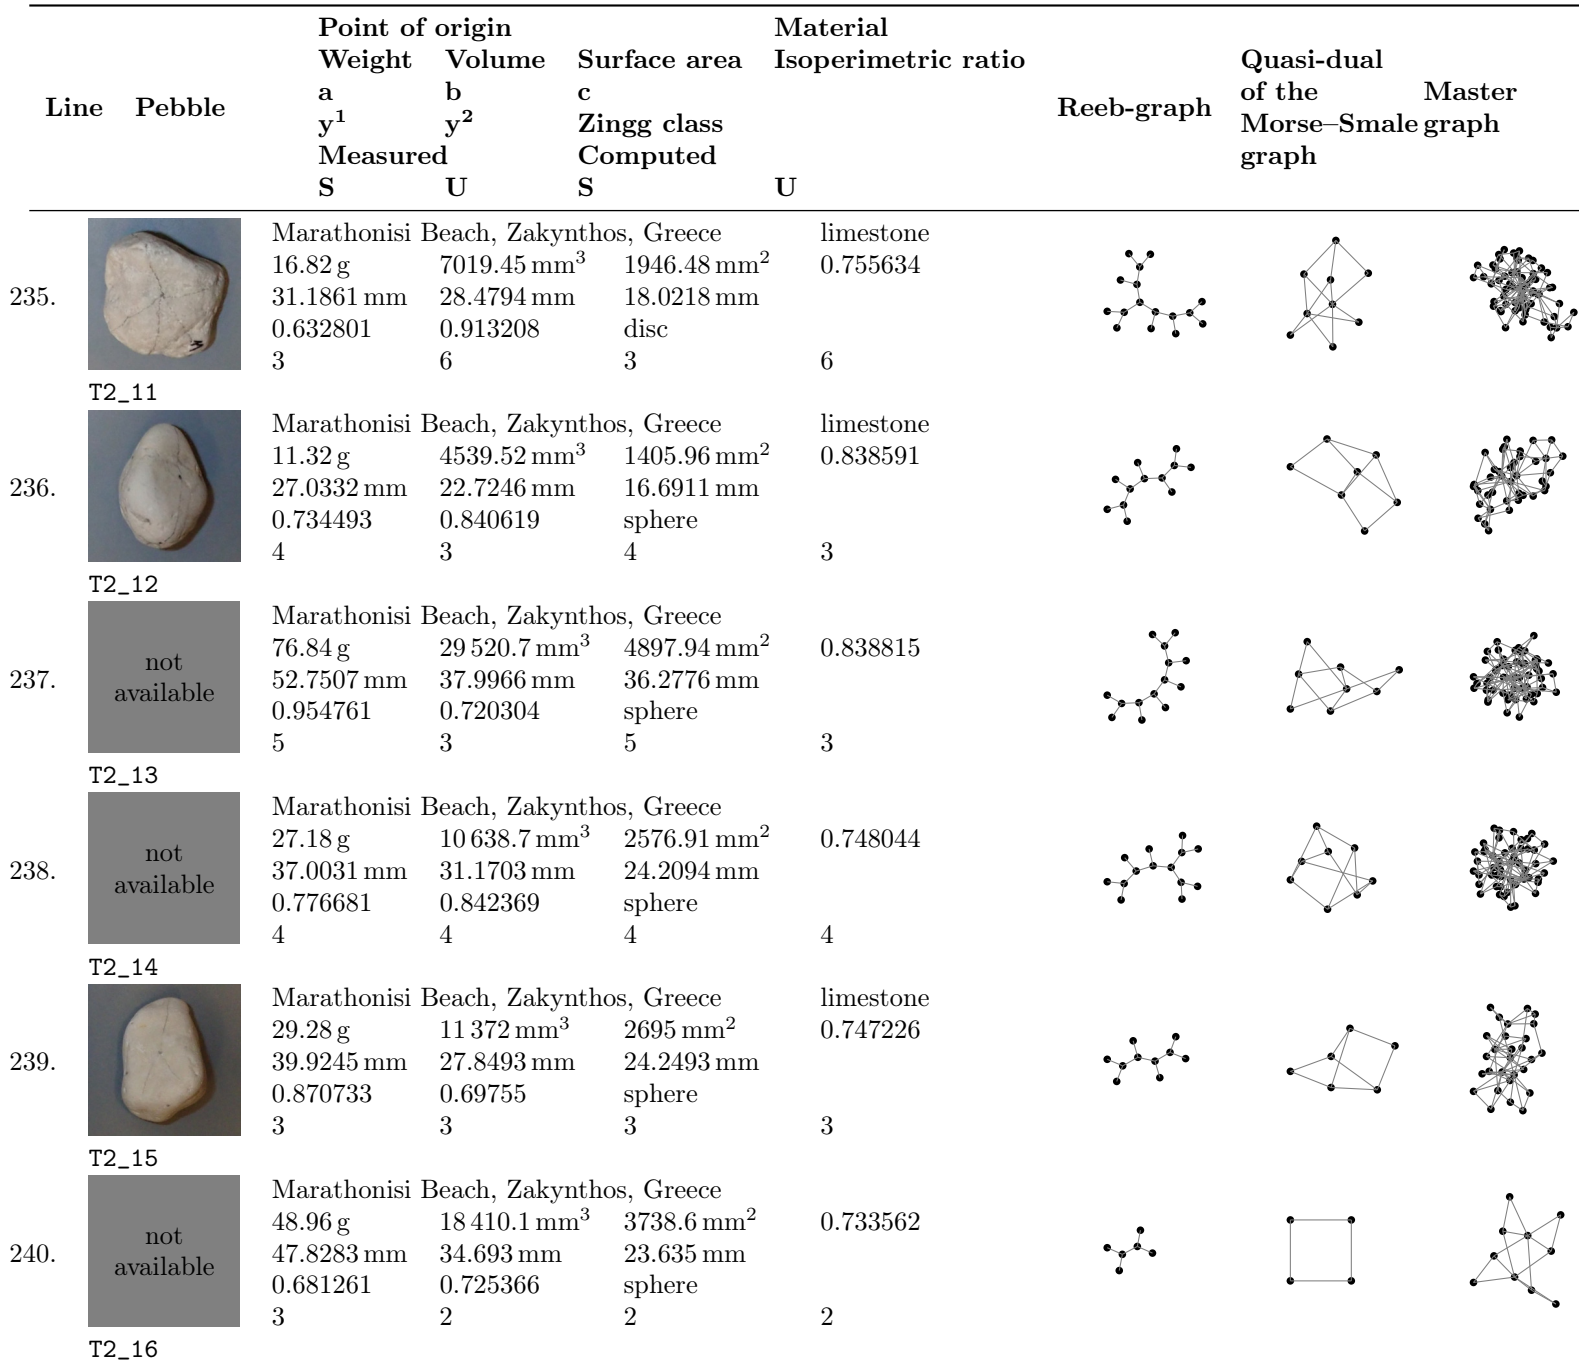   | 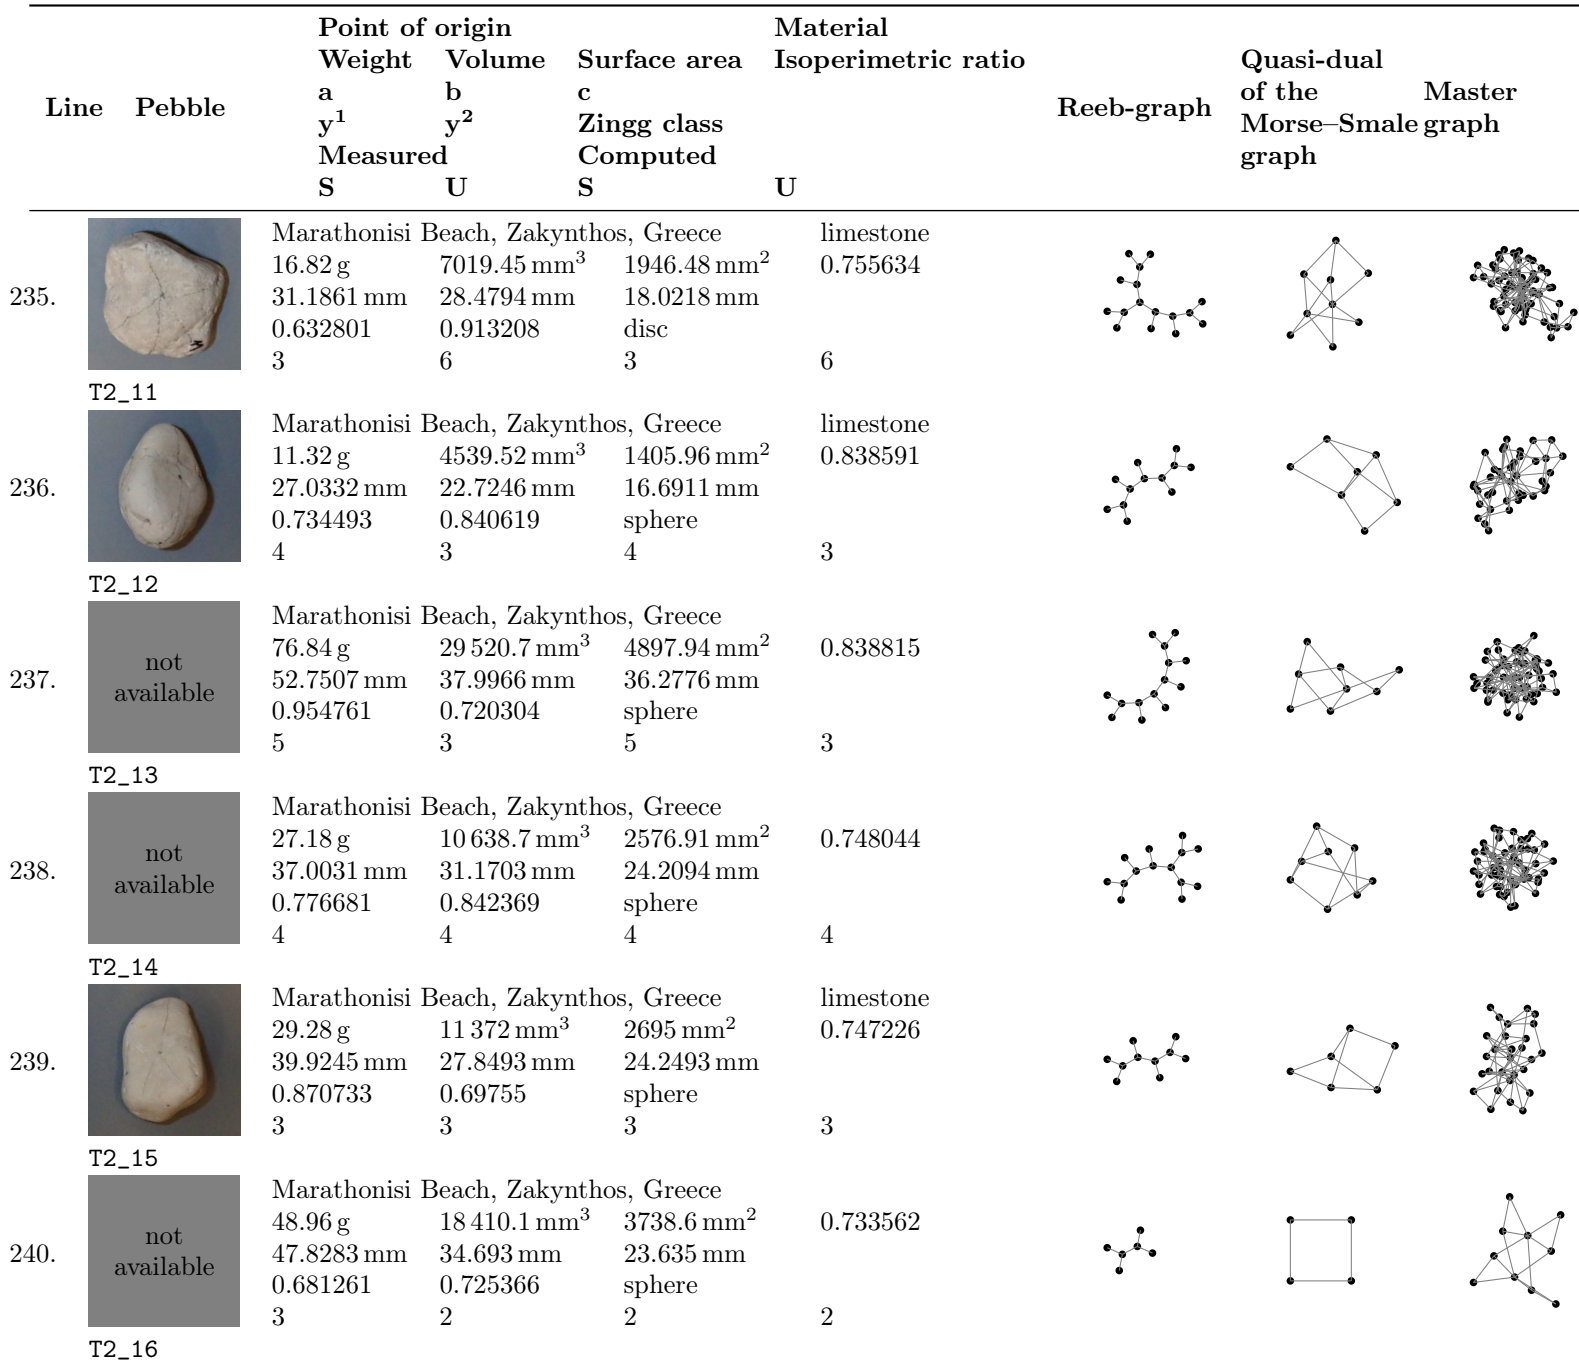   |
|      | T2_13                                                                               |                                                                                |                                                                                     |                                                      |                       |                                                                                       |                                                                                       |                                                                                       |
| 238. | 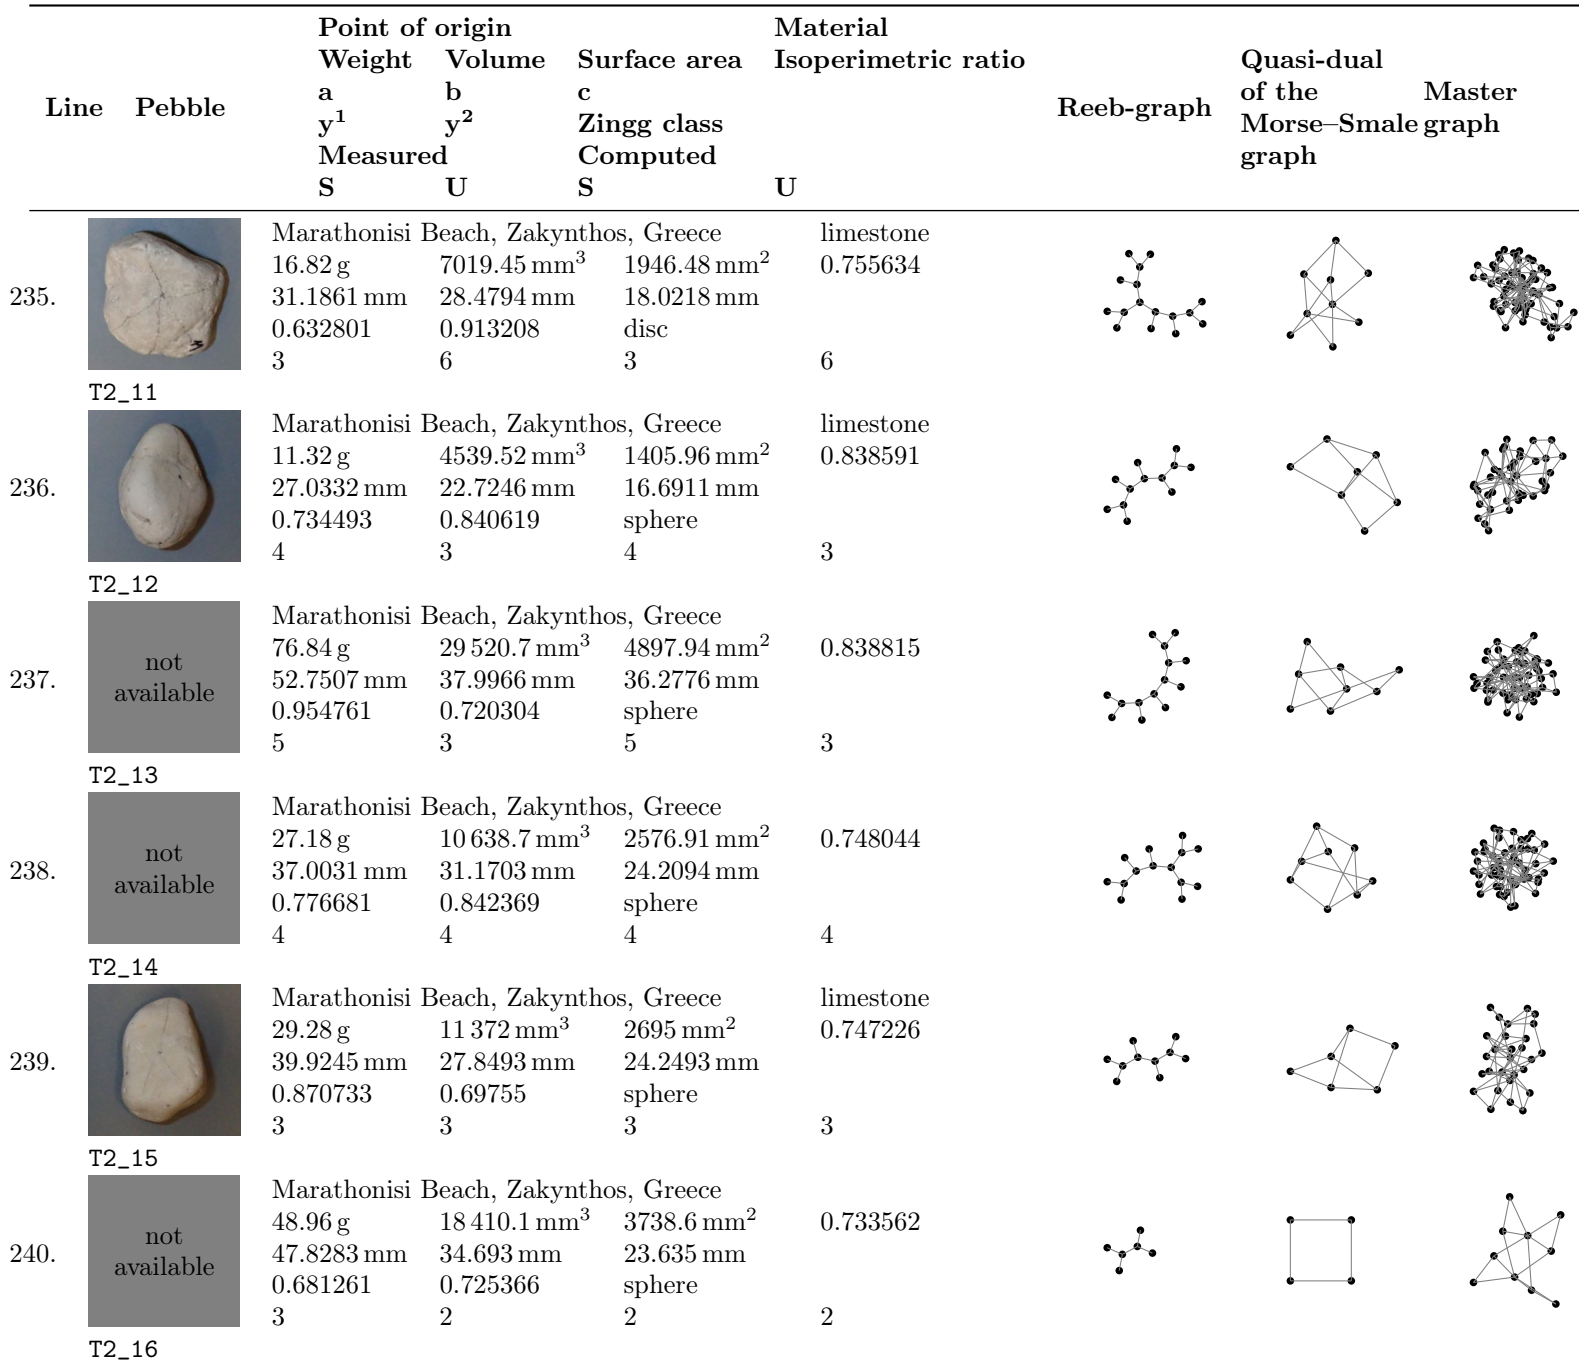  | Marathonisi Beach, Zakynthos, Greece<br>27.18 g<br>37.0031 mm<br>0.776681<br>4 | Beach, Zakynthos, Greece<br>10 638.7 mm <sup>3</sup><br>31.1703 mm<br>0.842369<br>4 | 2576.91 mm <sup>2</sup><br>24.2094 mm<br>sphere<br>4 | 0.748044              | 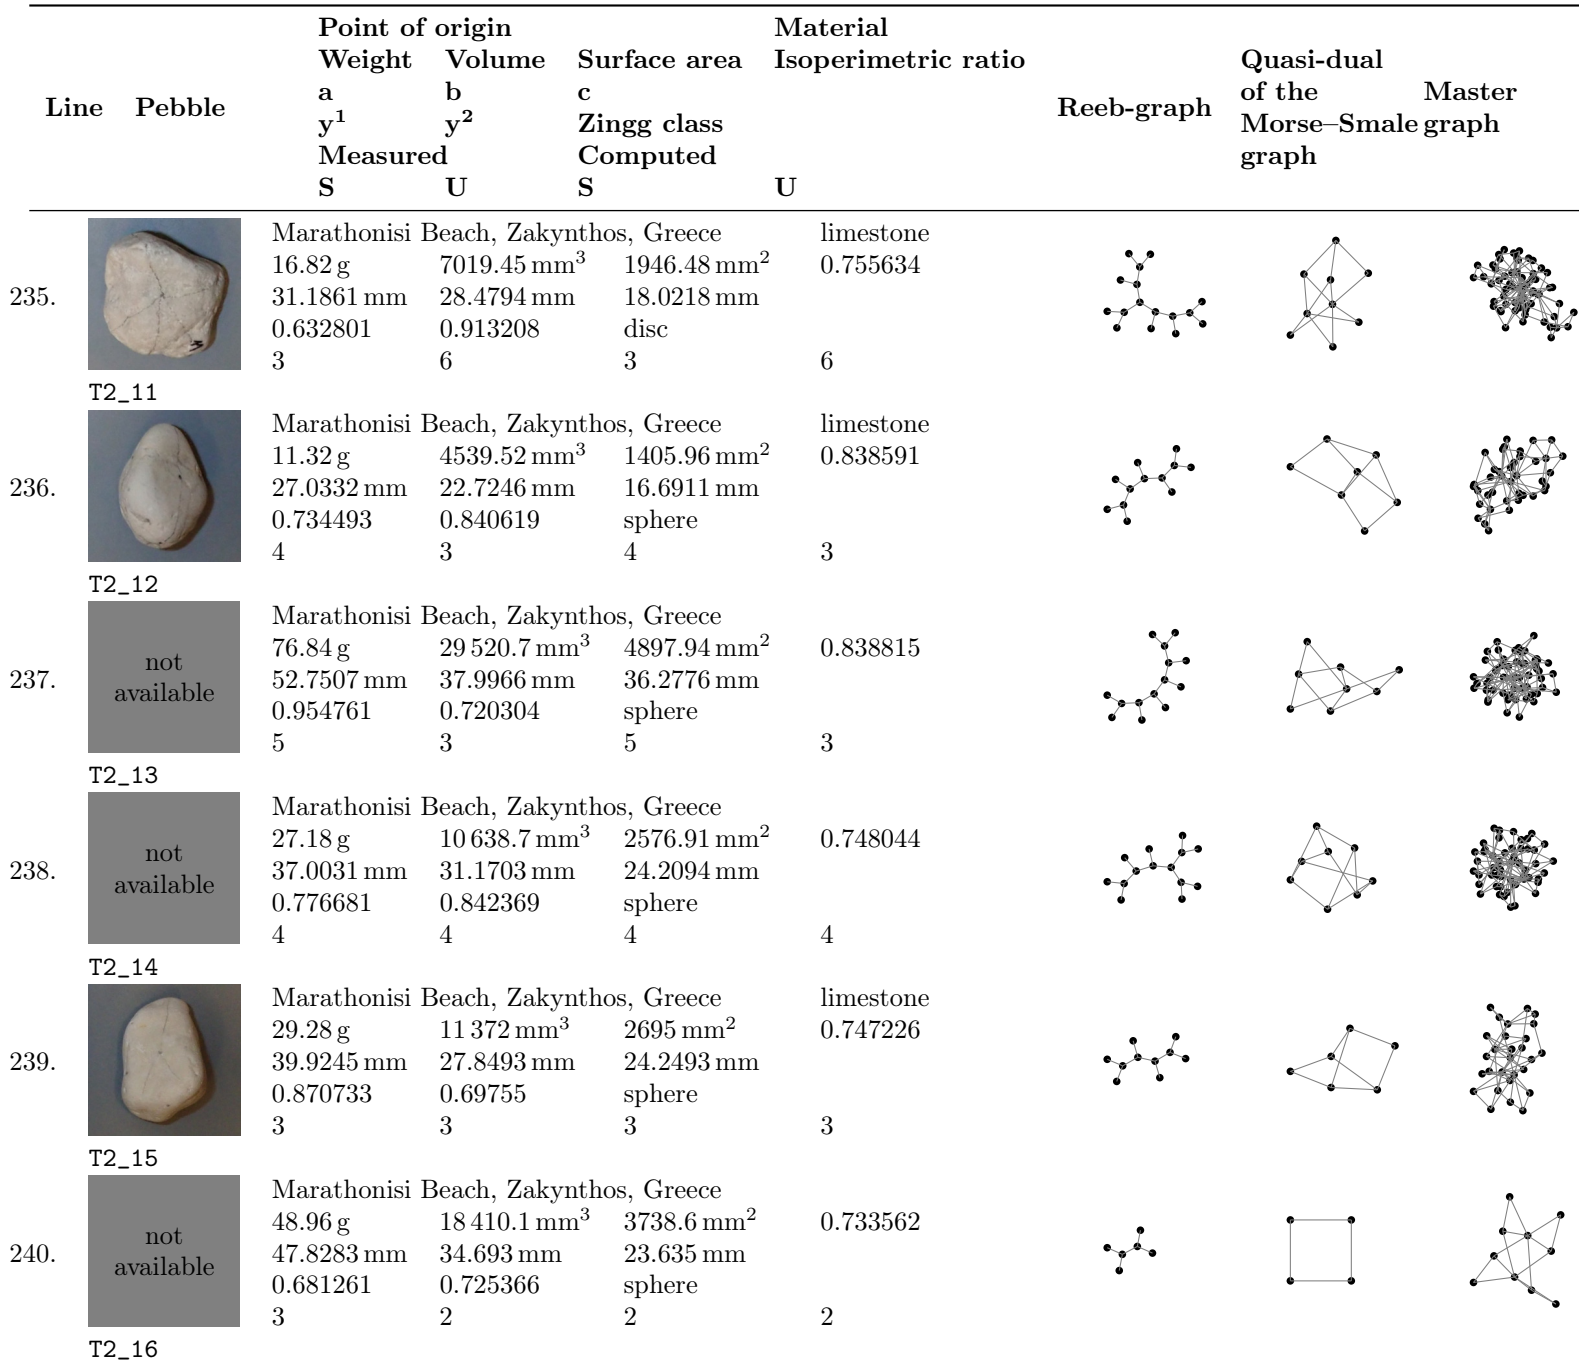  | 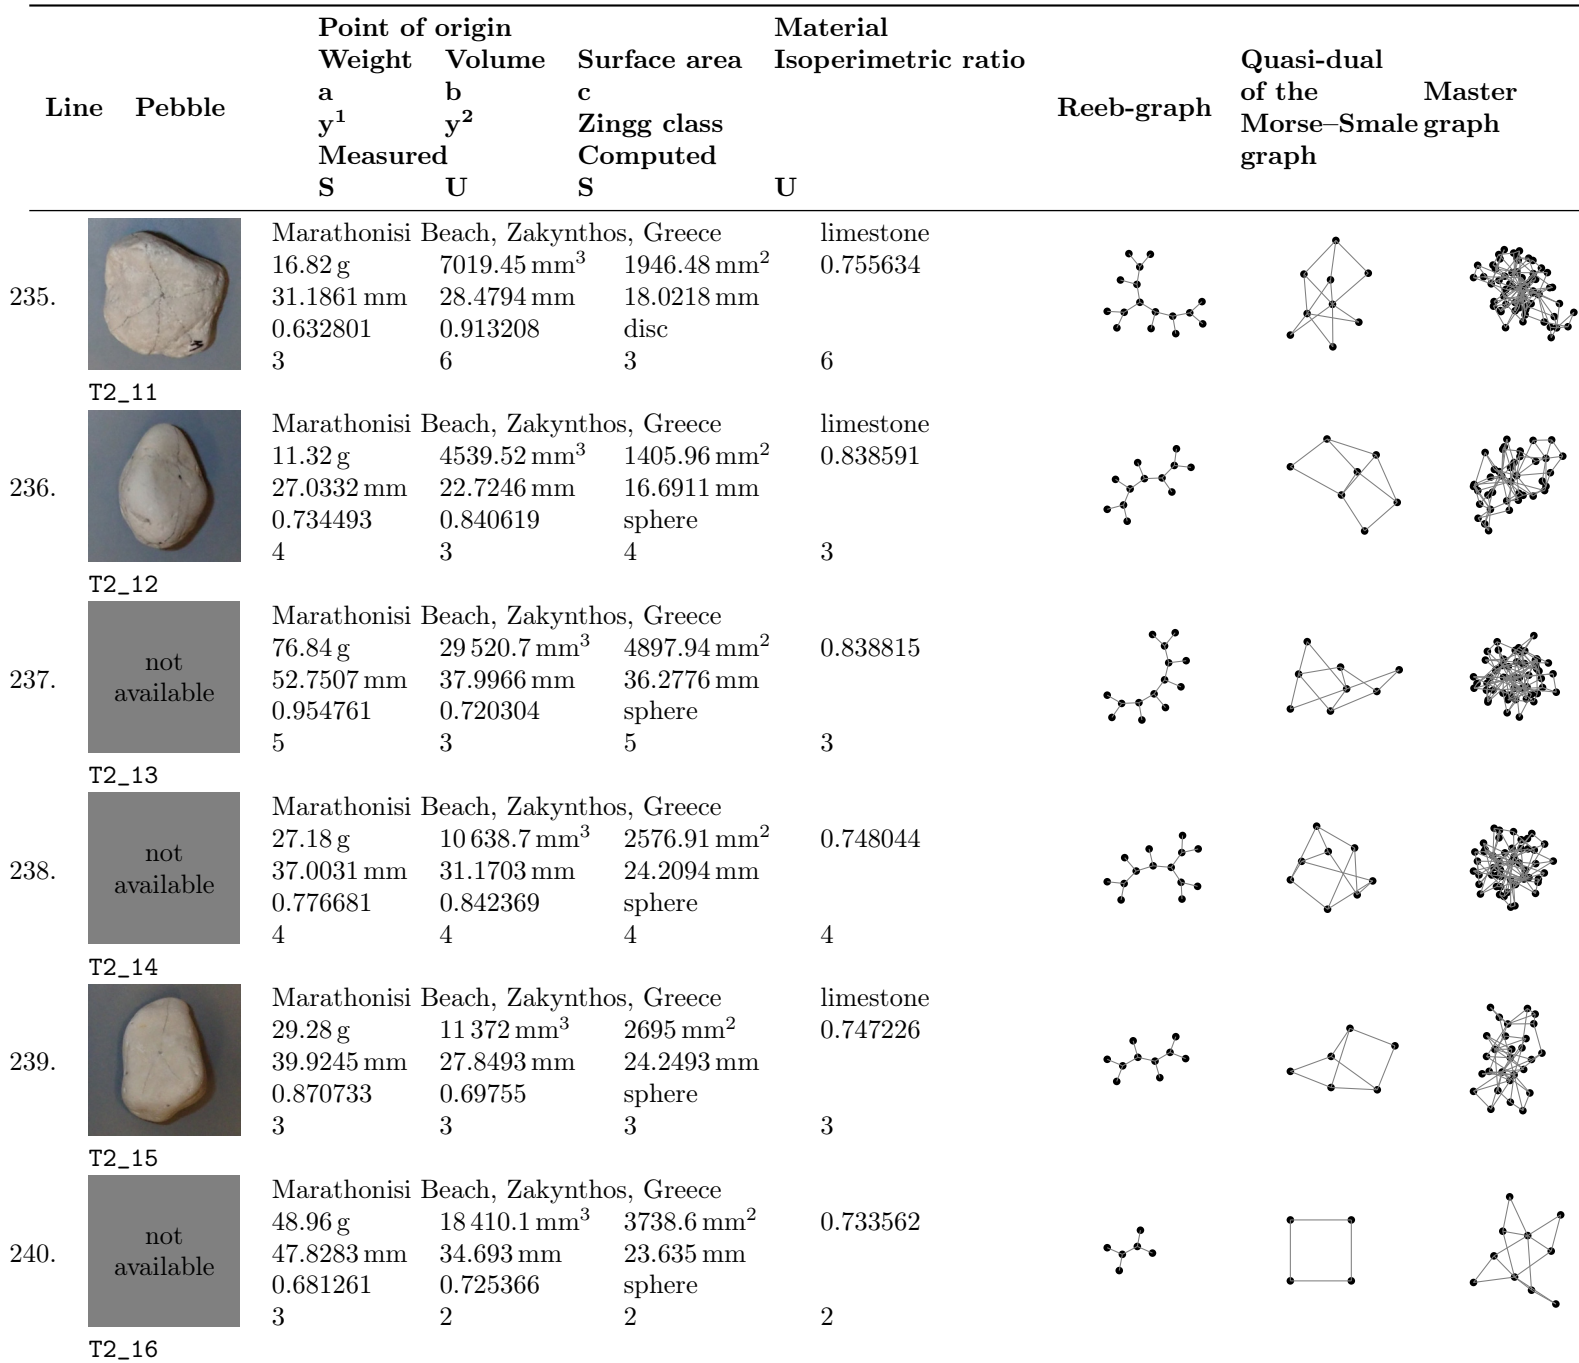  | 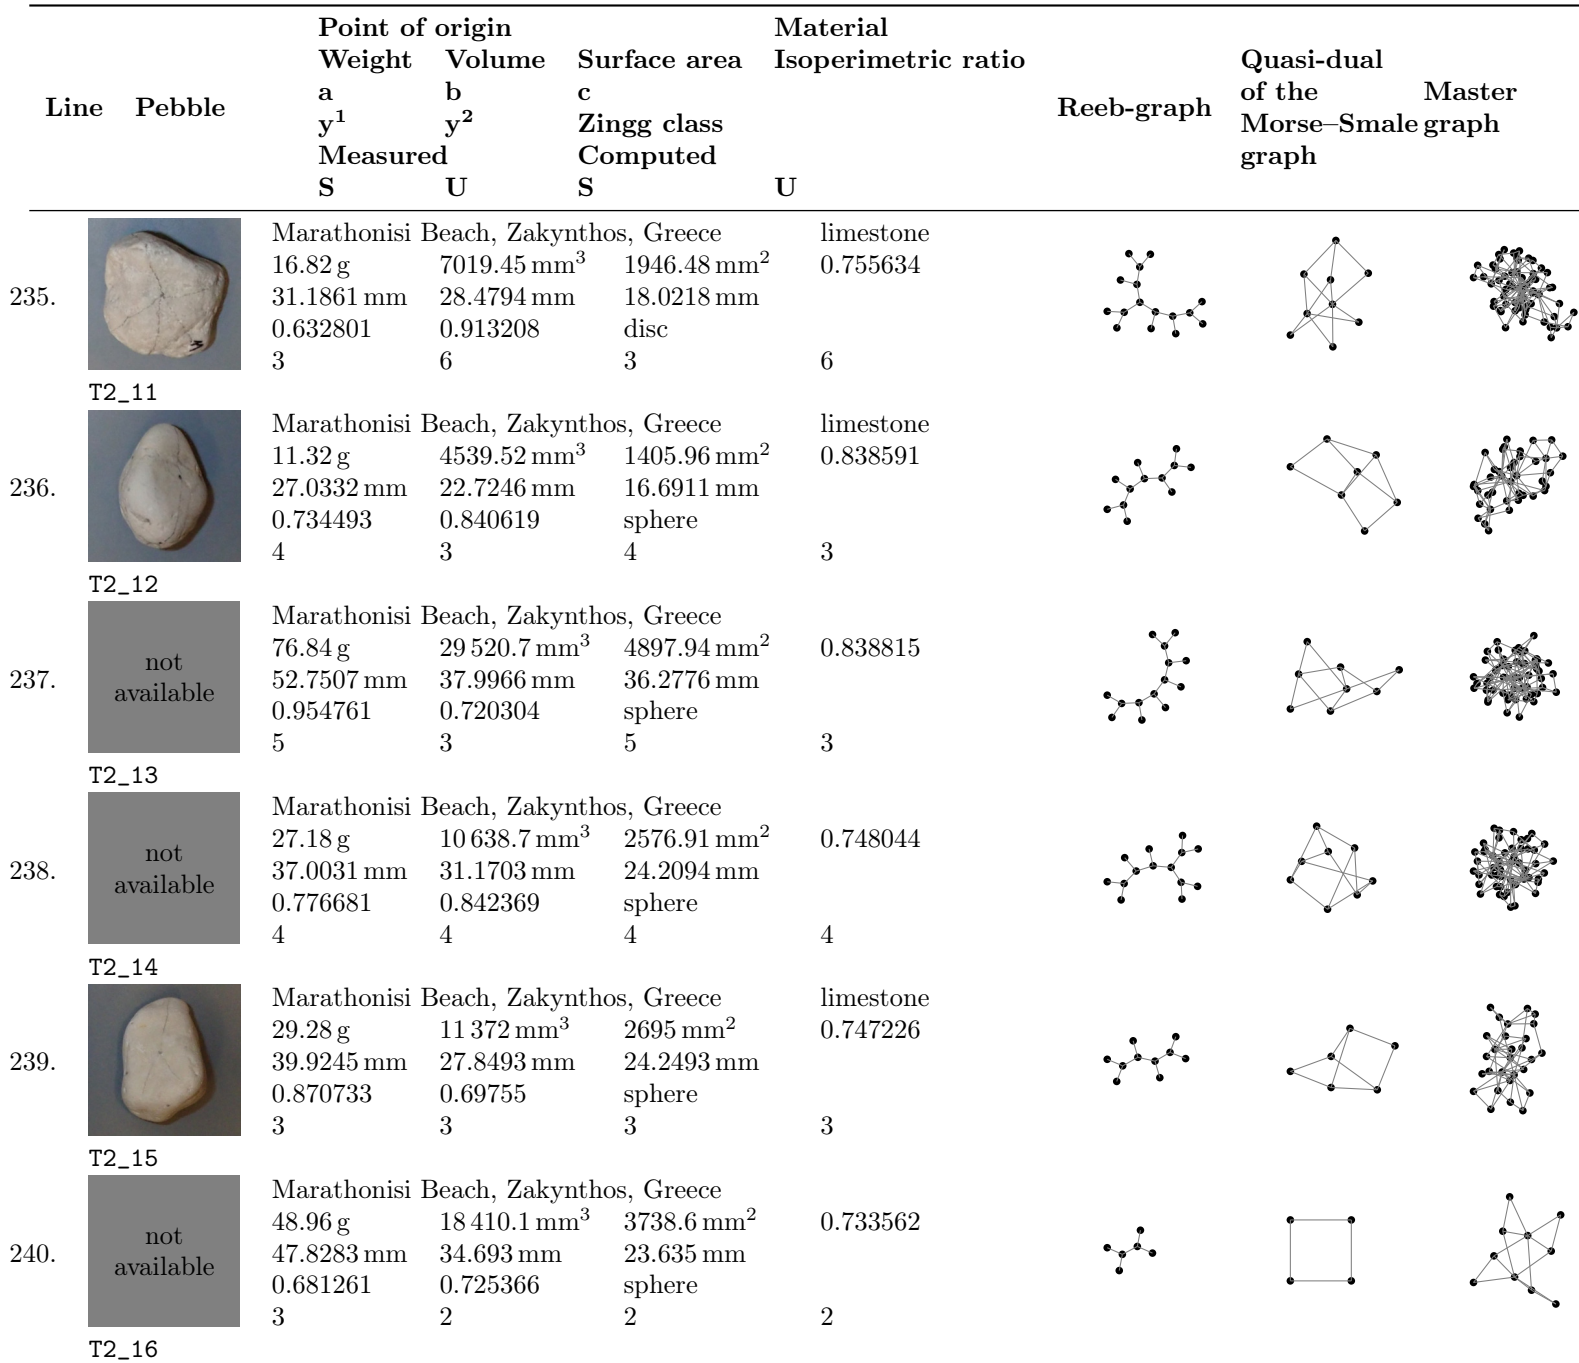  |
|      | T2_14                                                                               |                                                                                |                                                                                     |                                                      |                       |                                                                                       |                                                                                       |                                                                                       |
| 239. | 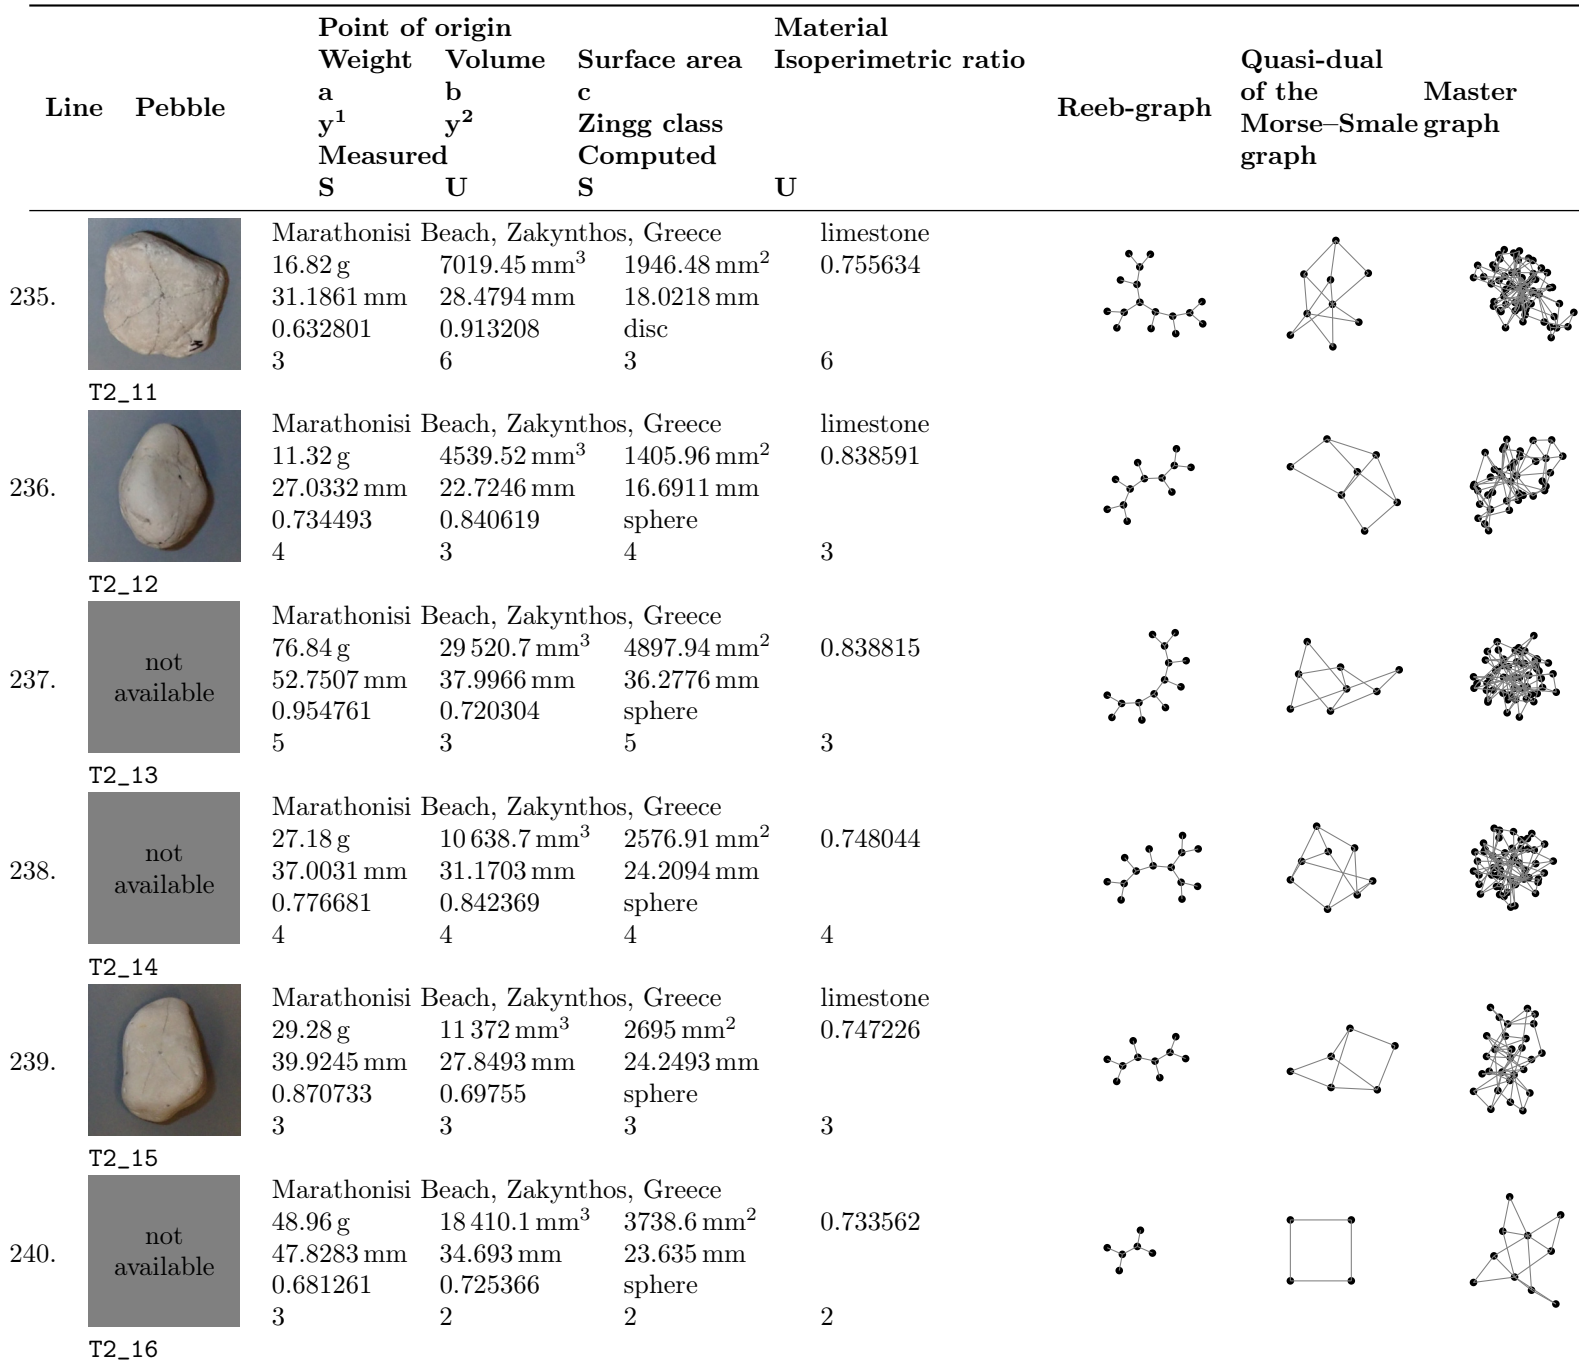 | Marathonisi Beach, Zakynthos, Greece<br>29.28 g<br>39.9245 mm<br>0.870733<br>3 | Beach, Zakynthos, Greece<br>11 372 mm <sup>3</sup><br>27.8493 mm<br>0.69755<br>3    | 2695 mm <sup>2</sup><br>24.2493 mm<br>sphere<br>3    | limestone<br>0.747226 | 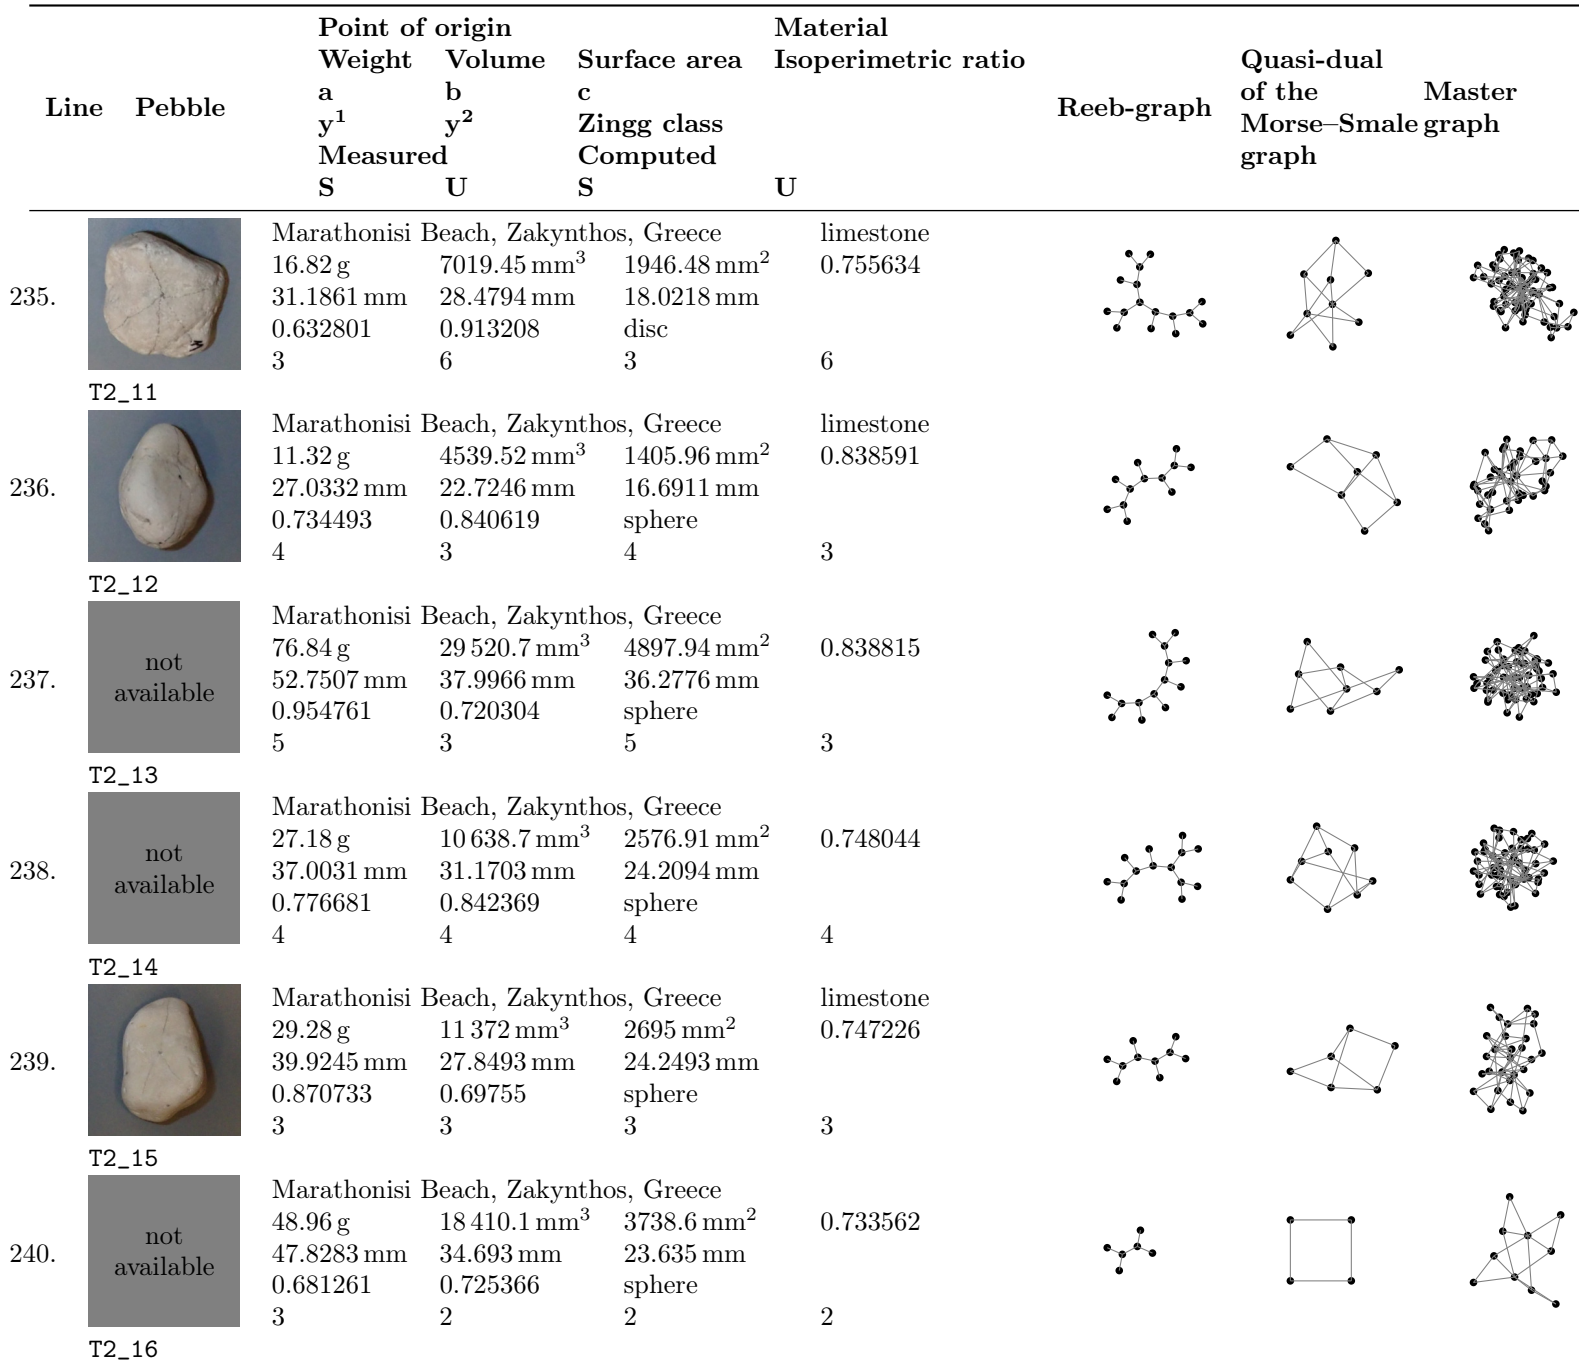 | 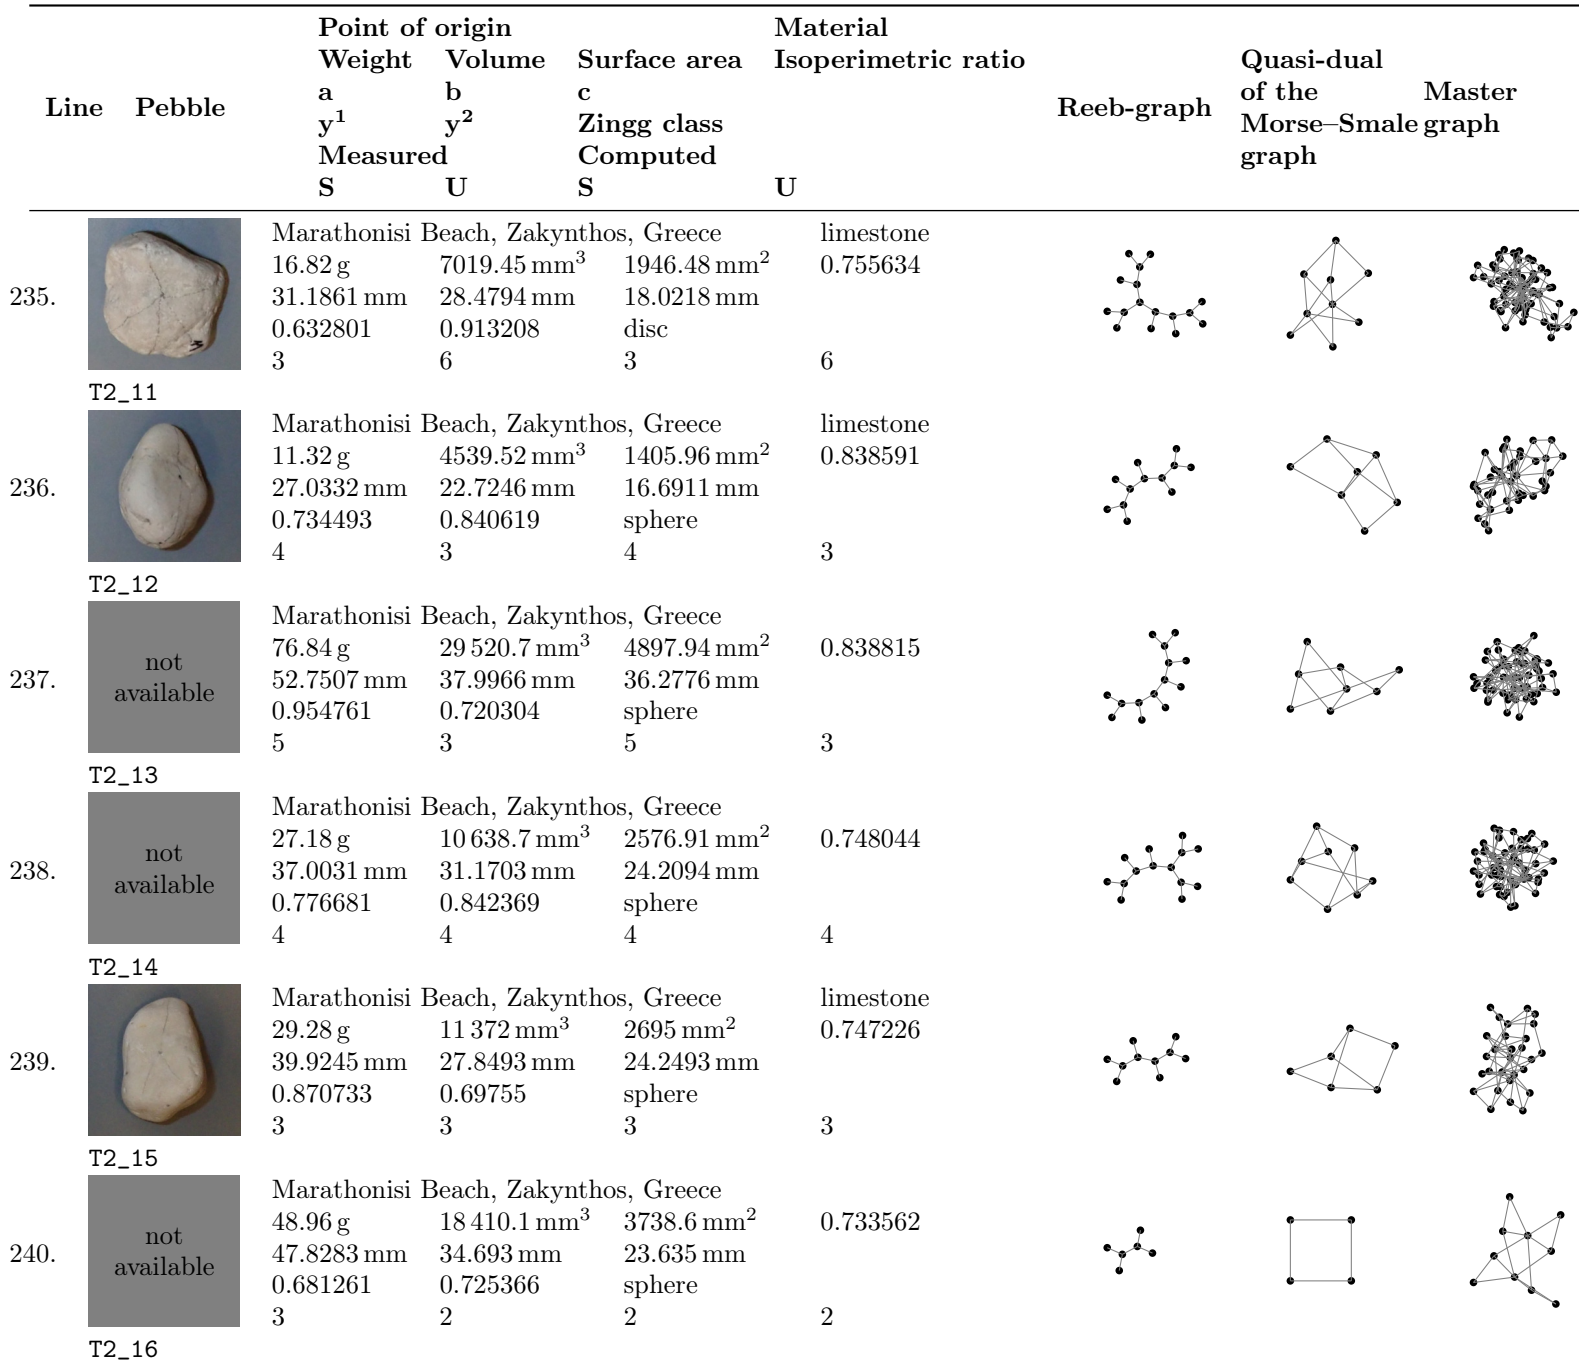 | 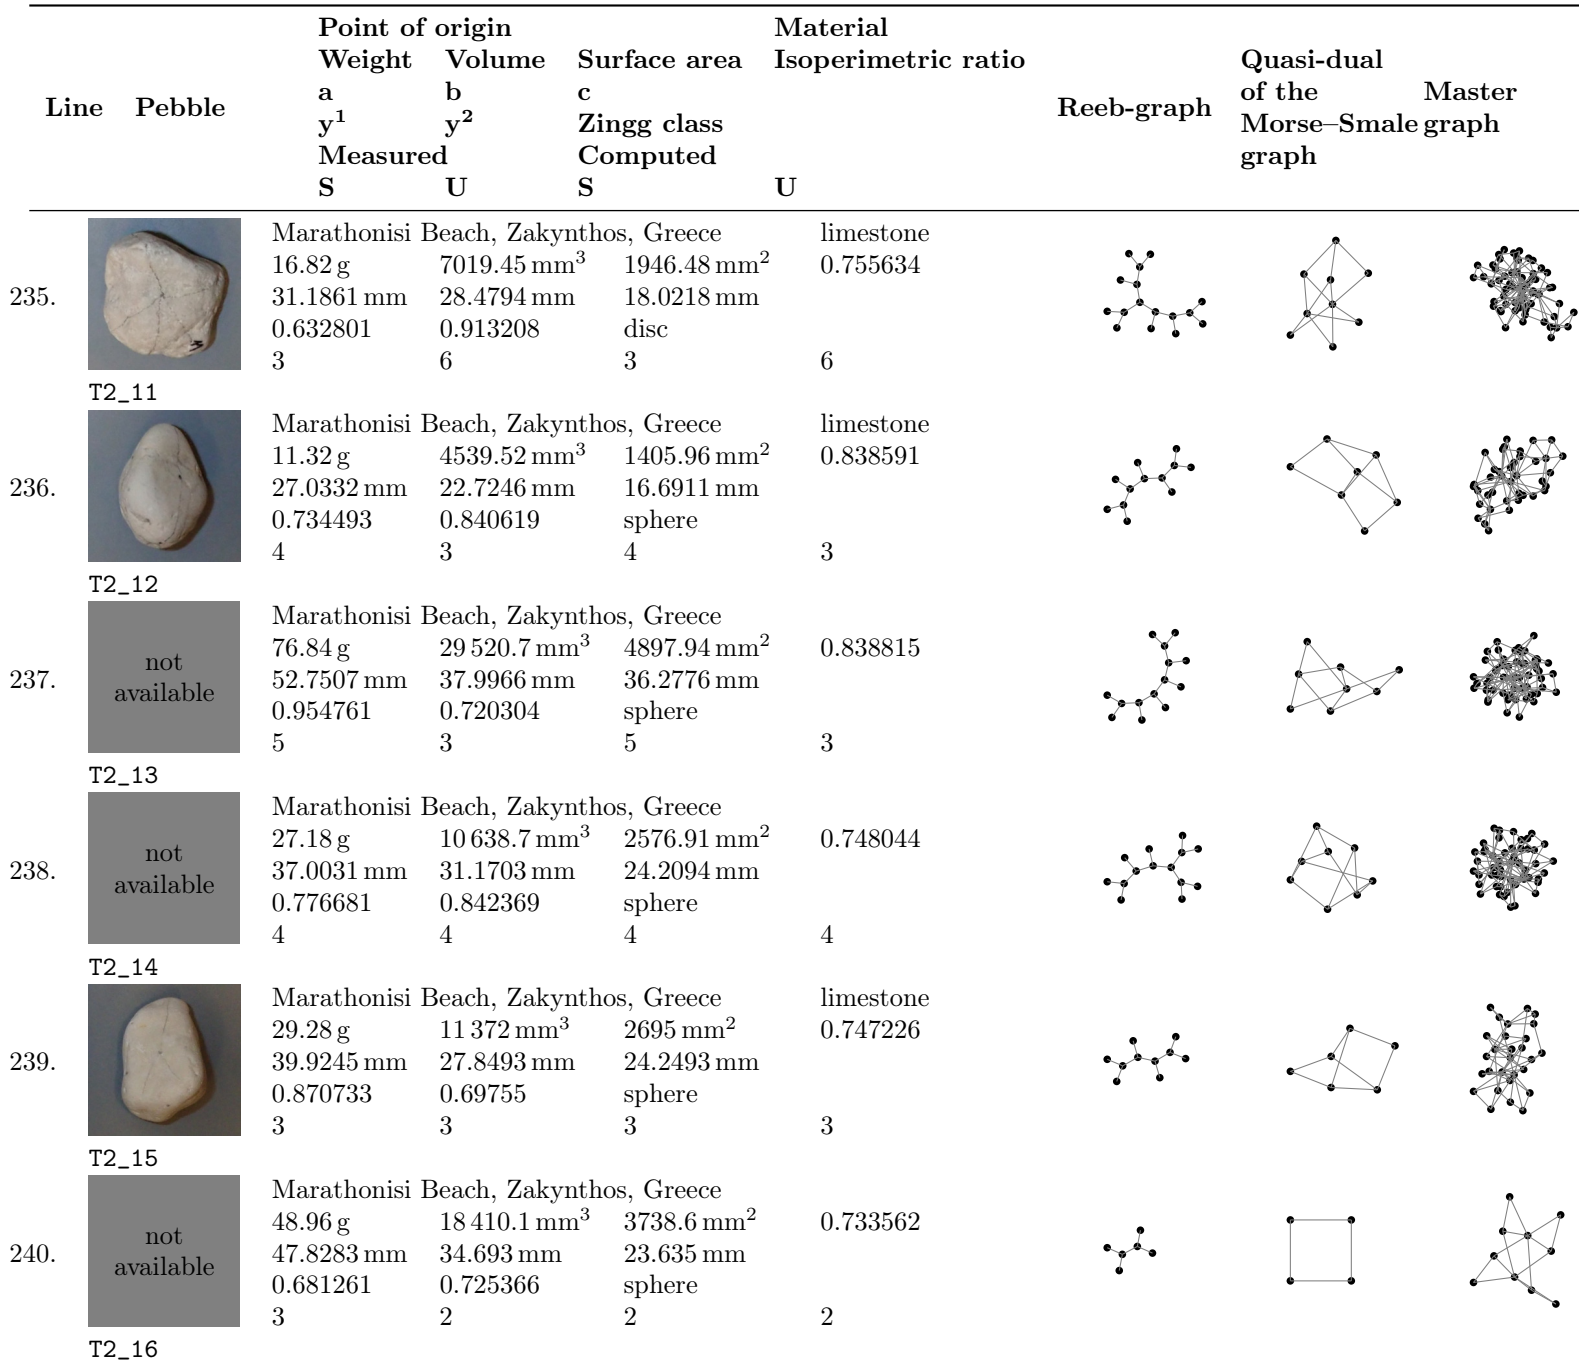 |
|      | T2_15                                                                               |                                                                                |                                                                                     |                                                      |                       |                                                                                       |                                                                                       |                                                                                       |
| 240. | 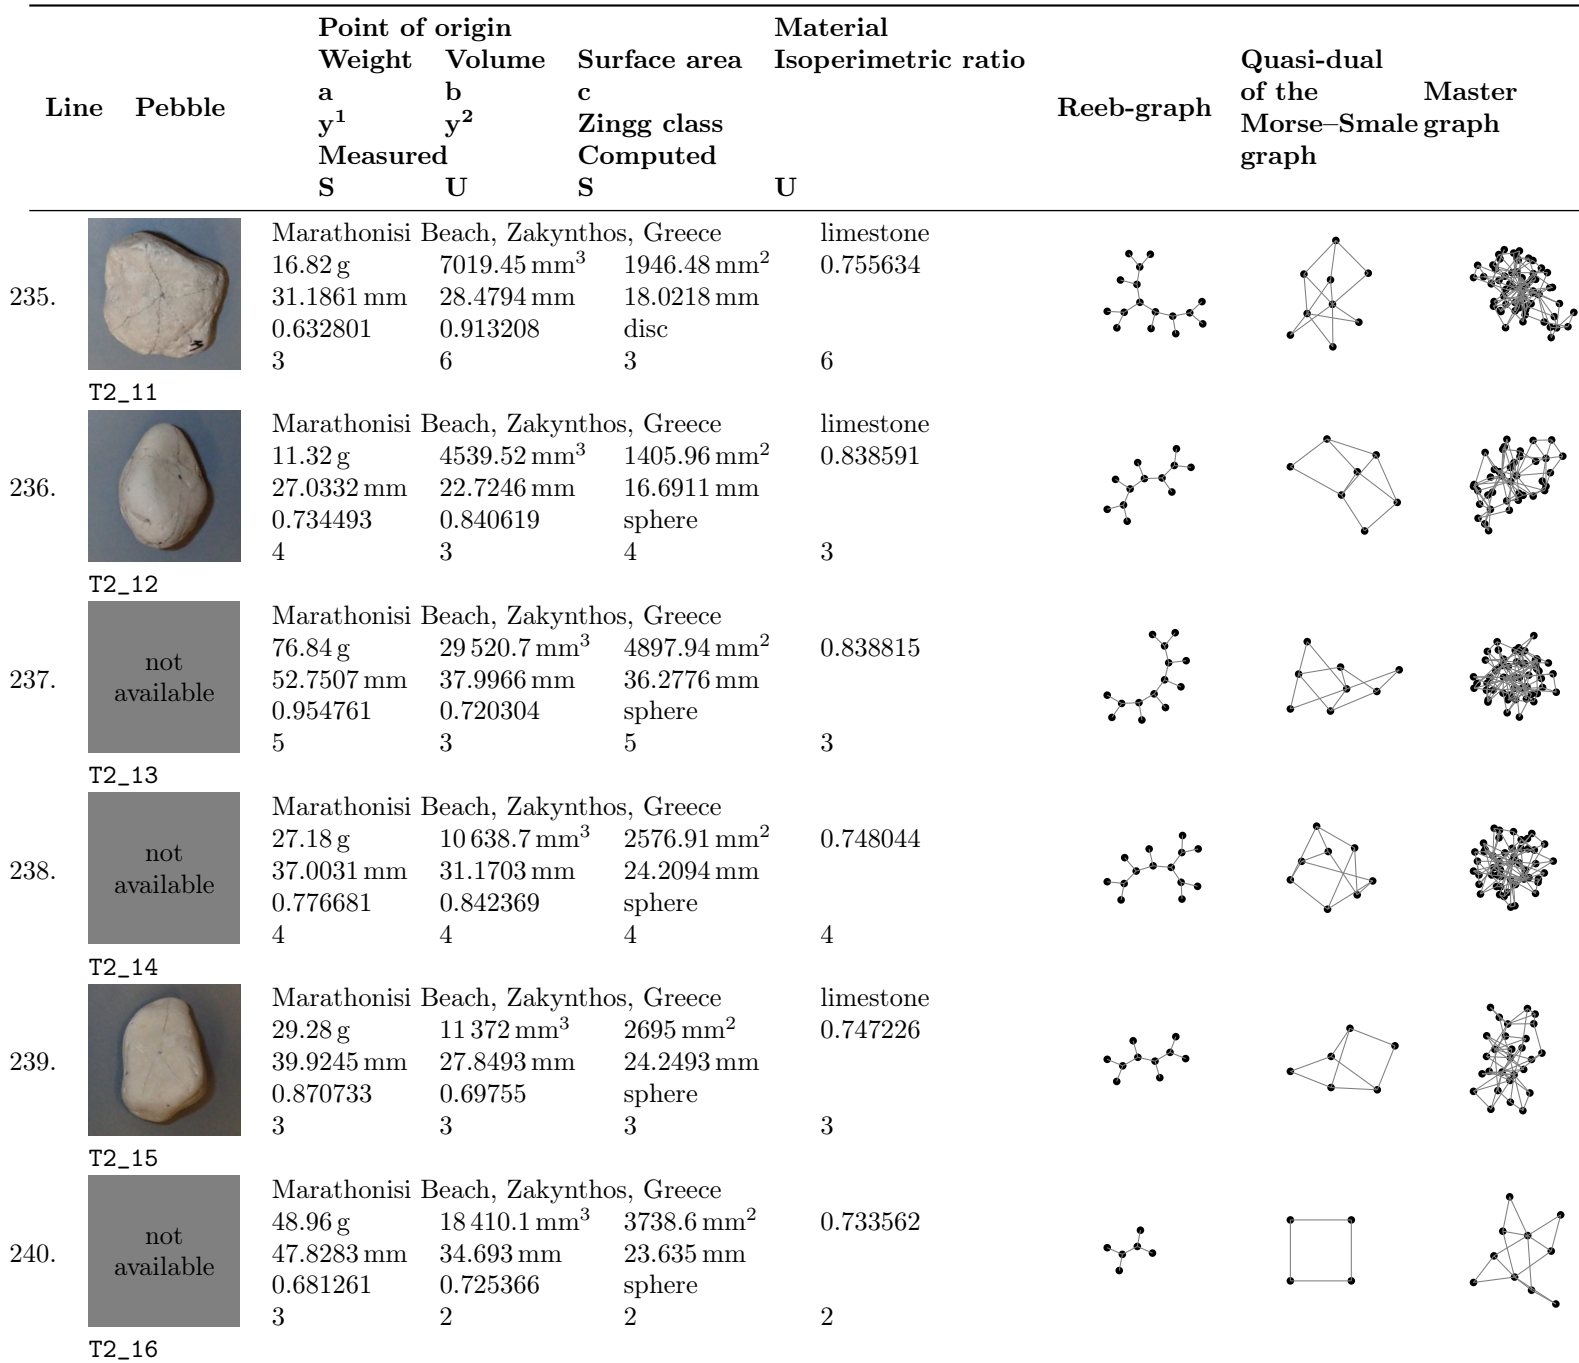 | Marathonisi Beach, Zakynthos, Greece<br>48.96 g<br>47.8283 mm<br>0.681261<br>3 | Beach, Zakynthos, Greece<br>18 410.1 mm <sup>3</sup><br>34.693 mm<br>0.725366<br>2  | 3738.6 mm <sup>2</sup><br>23.635 mm<br>sphere<br>2   | 0.733562              | 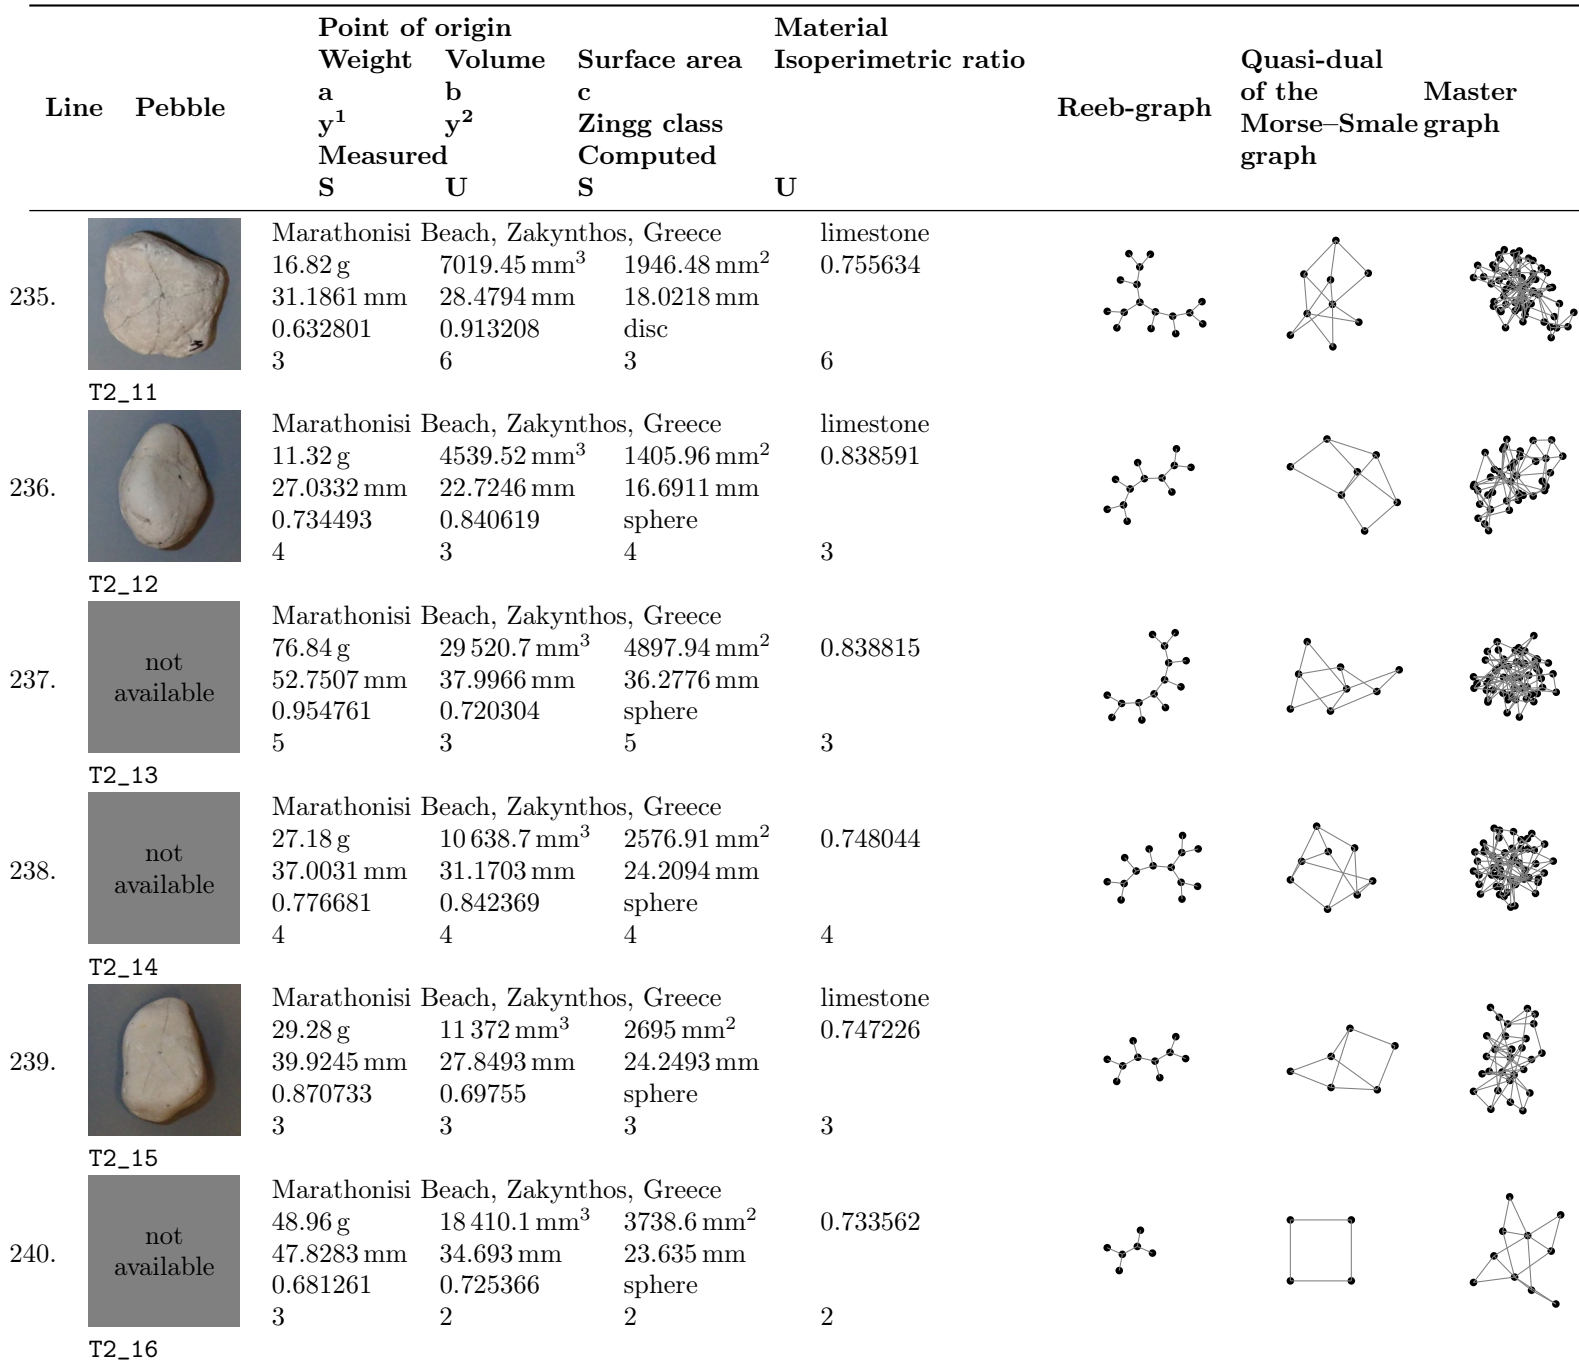 | 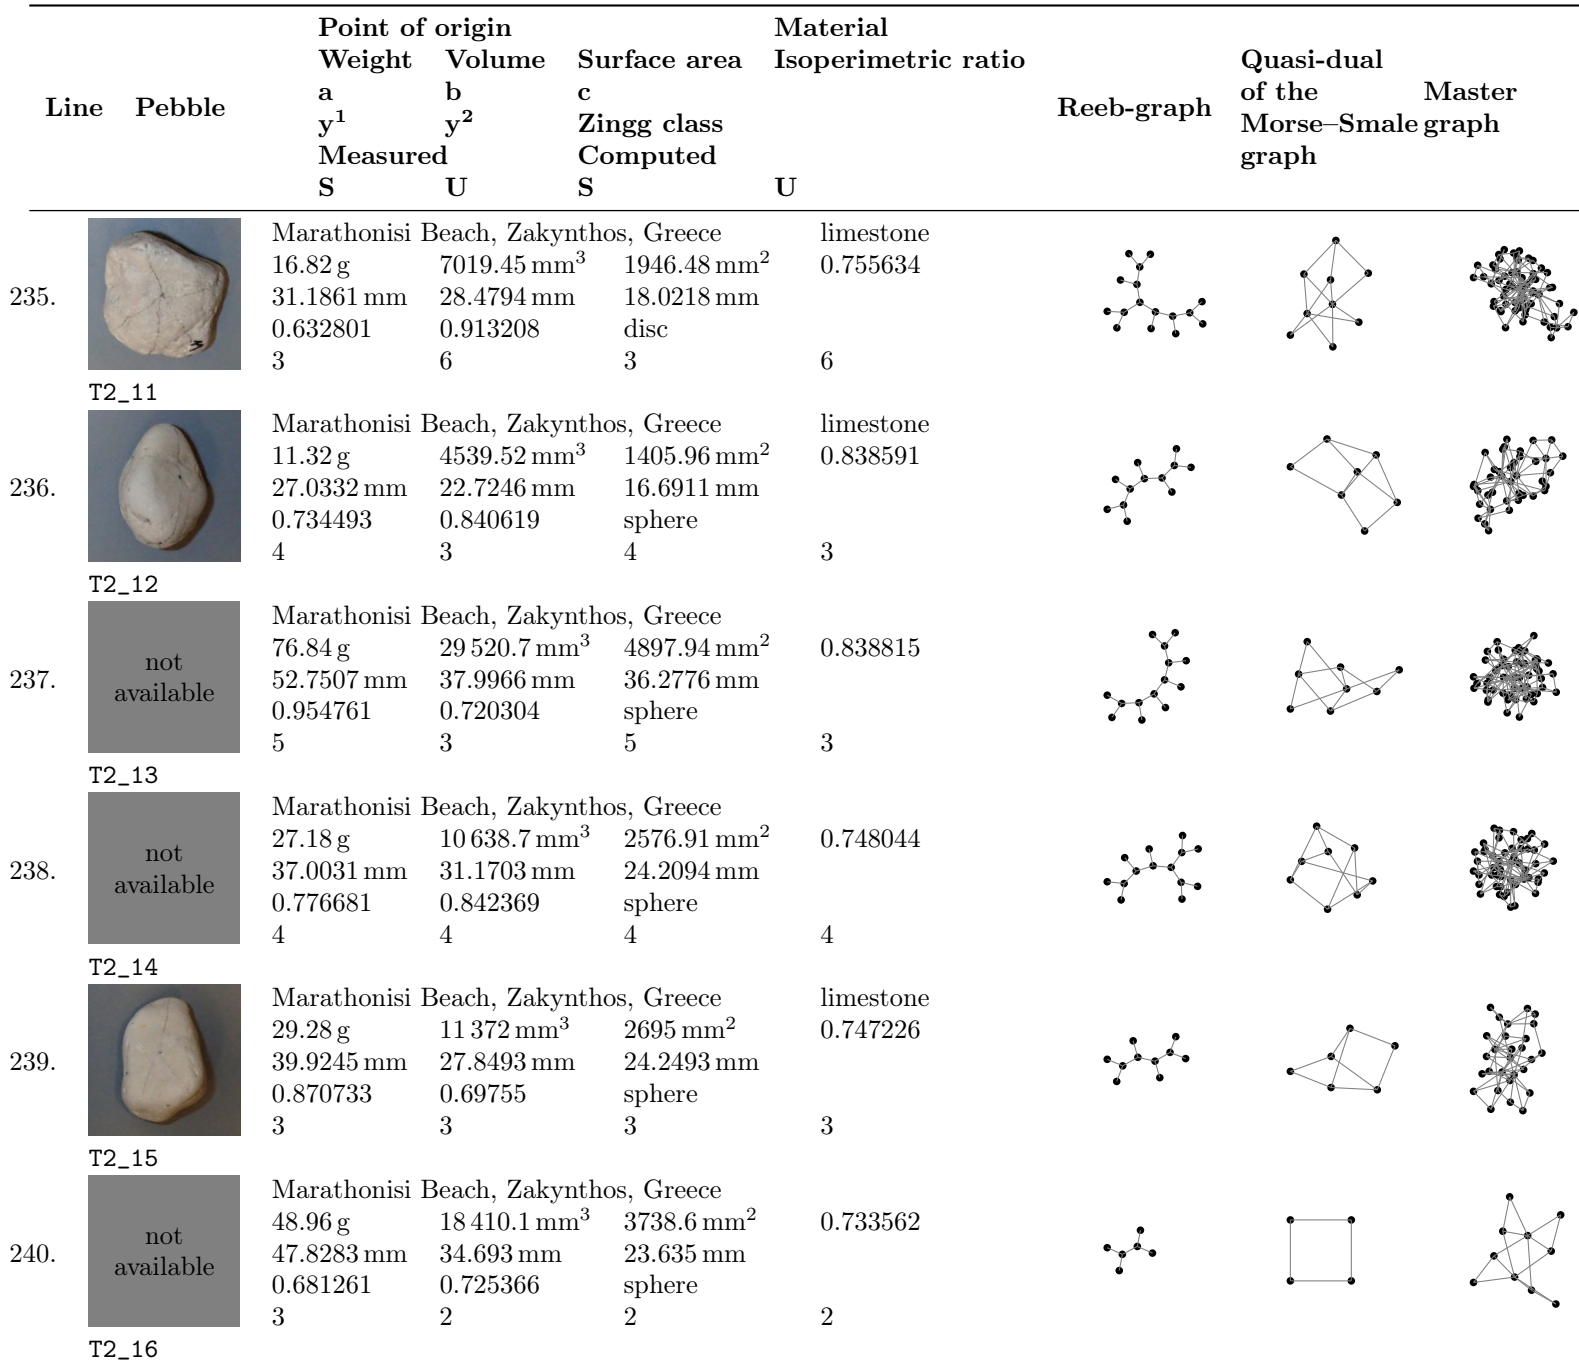 | 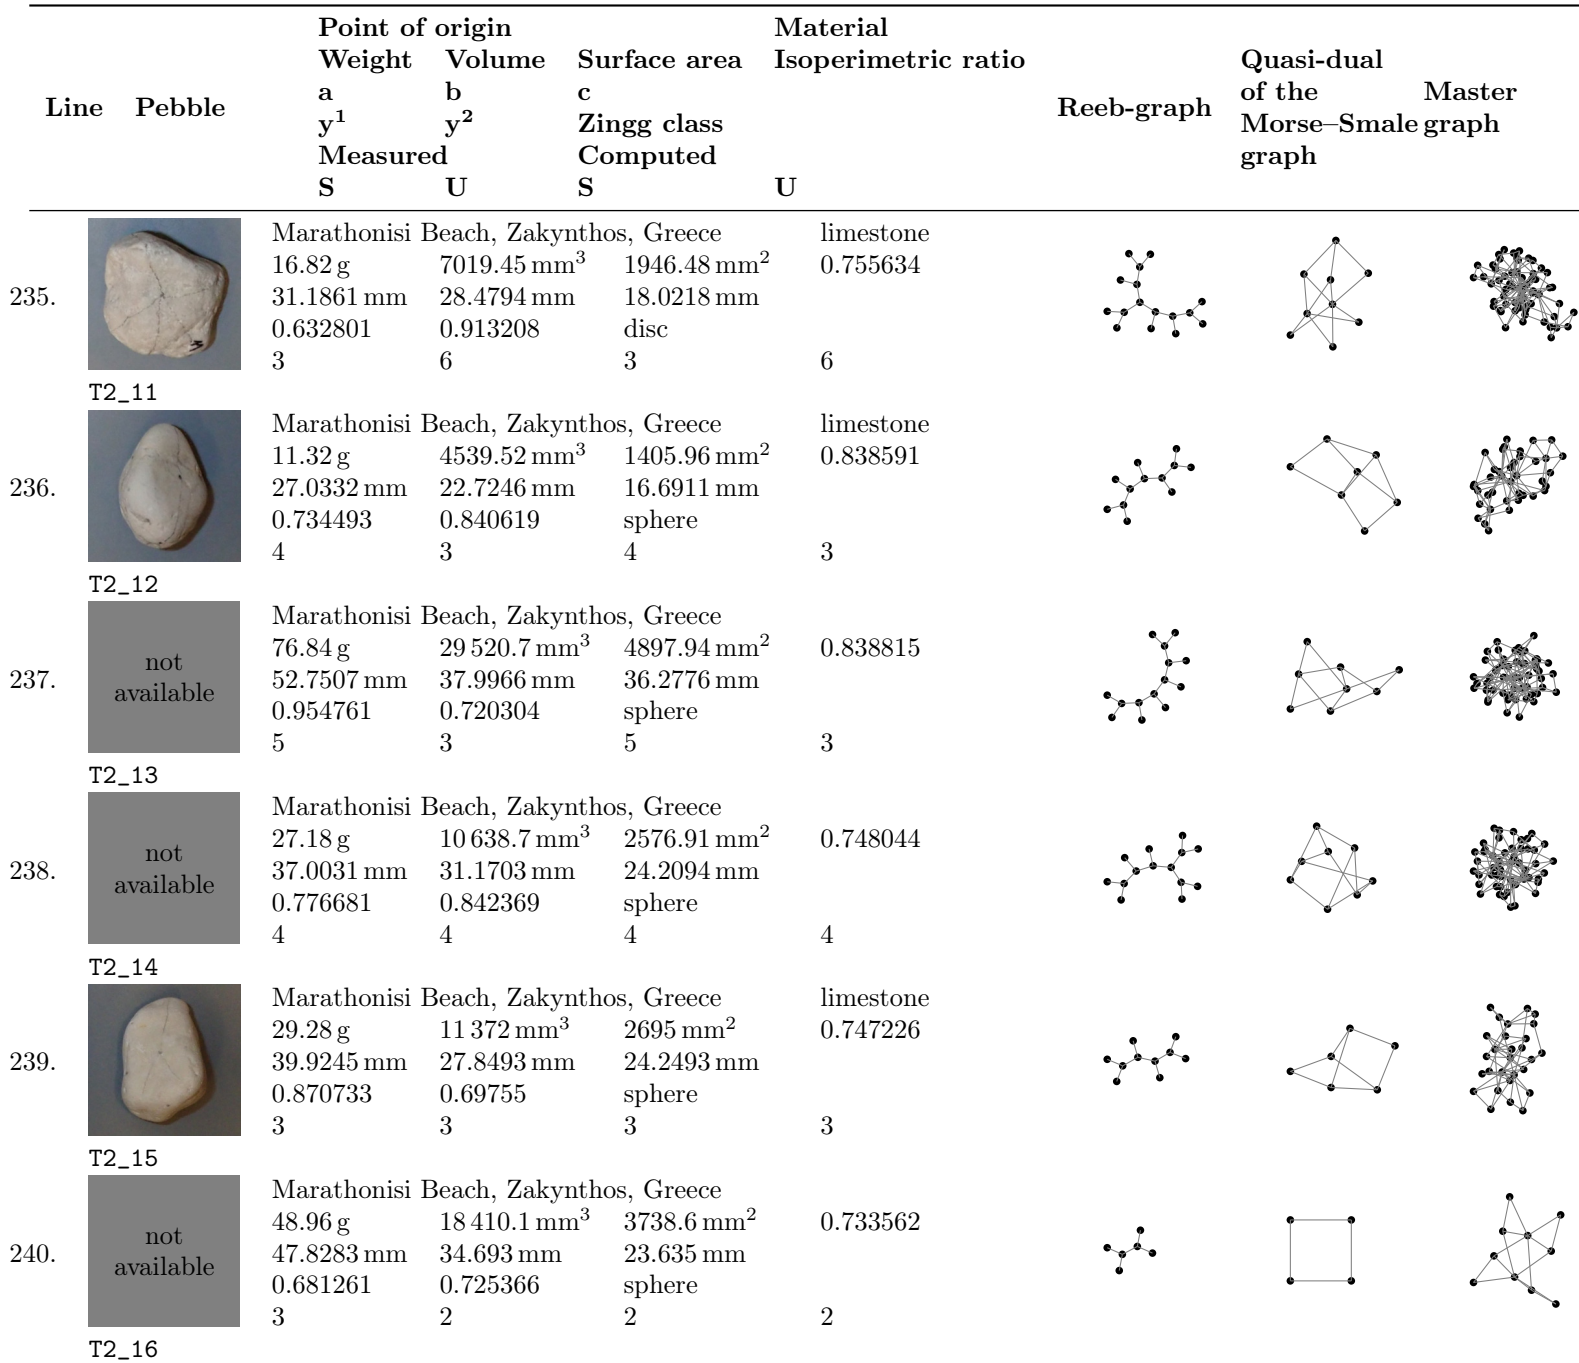 |
|      | T2_16                                                                               |                                                                                |                                                                                     |                                                      |                       |                                                                                       |                                                                                       |                                                                                       |

| Line | Pebble                                                                              | Point of origin                                                                |                                                         | Surface area<br>c<br>Zingg class<br>Computed<br>S    | Material<br>Isoperimetric ratio<br>U | Reeb-graph                                                                            | Quasi-dual<br>of the<br>Morse–Smale<br>graph                                          | Master<br>graph                                                                       |
|------|-------------------------------------------------------------------------------------|--------------------------------------------------------------------------------|---------------------------------------------------------|------------------------------------------------------|--------------------------------------|---------------------------------------------------------------------------------------|---------------------------------------------------------------------------------------|---------------------------------------------------------------------------------------|
|      |                                                                                     | Weight                                                                         | Volume                                                  |                                                      |                                      |                                                                                       |                                                                                       |                                                                                       |
|      |                                                                                     | a<br>y <sup>1</sup><br>Measured<br>S                                           | b<br>y <sup>2</sup><br>U                                |                                                      |                                      |                                                                                       |                                                                                       |                                                                                       |
|      |                                                                                     |                                                                                |                                                         |                                                      |                                      |                                                                                       |                                                                                       |                                                                                       |
| 241. | 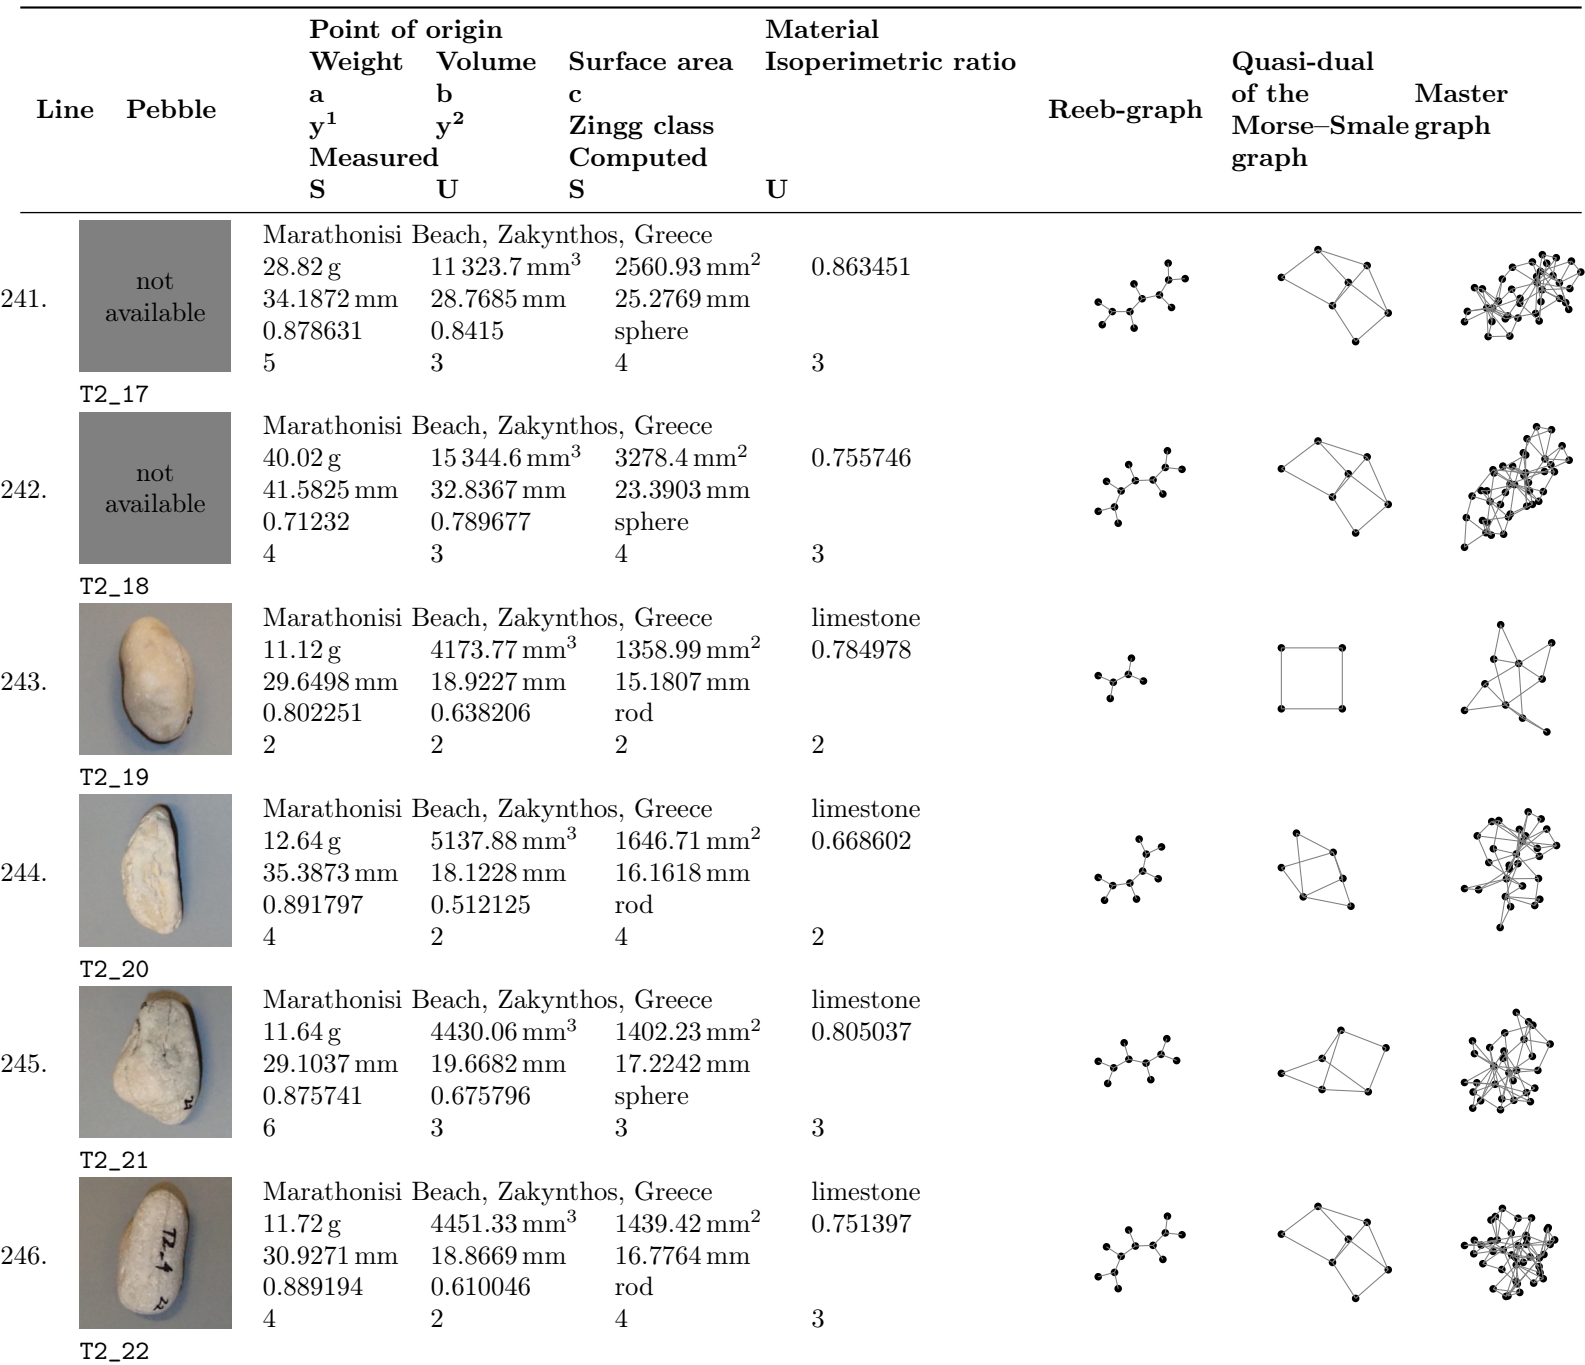   | Marathonisi Beach, Zakynthos, Greece<br>28.82 g<br>34.1872 mm<br>0.878631<br>5 | 11 323.7 mm <sup>3</sup><br>28.7685 mm<br>0.8415<br>3   | 2560.93 mm <sup>2</sup><br>25.2769 mm<br>sphere<br>4 | 0.863451<br><br><br>3                | 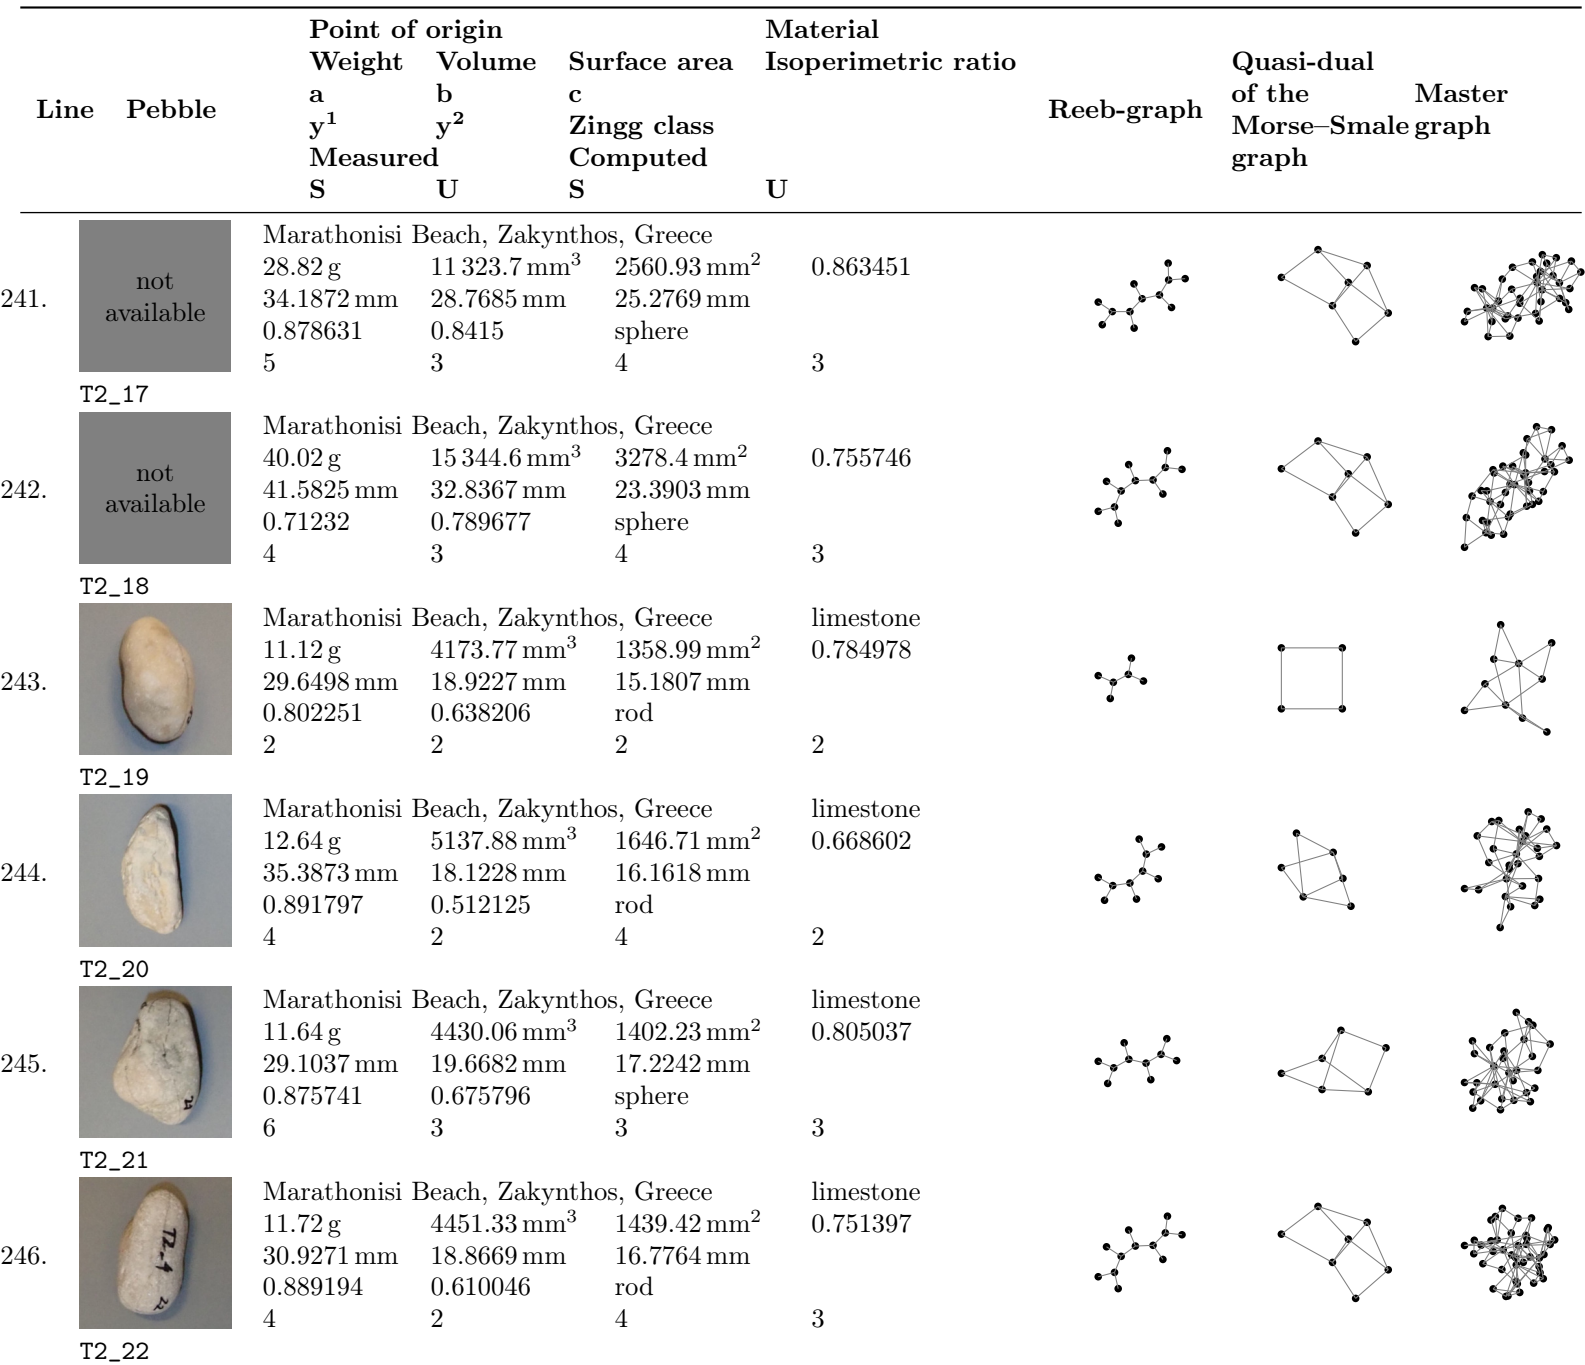   | 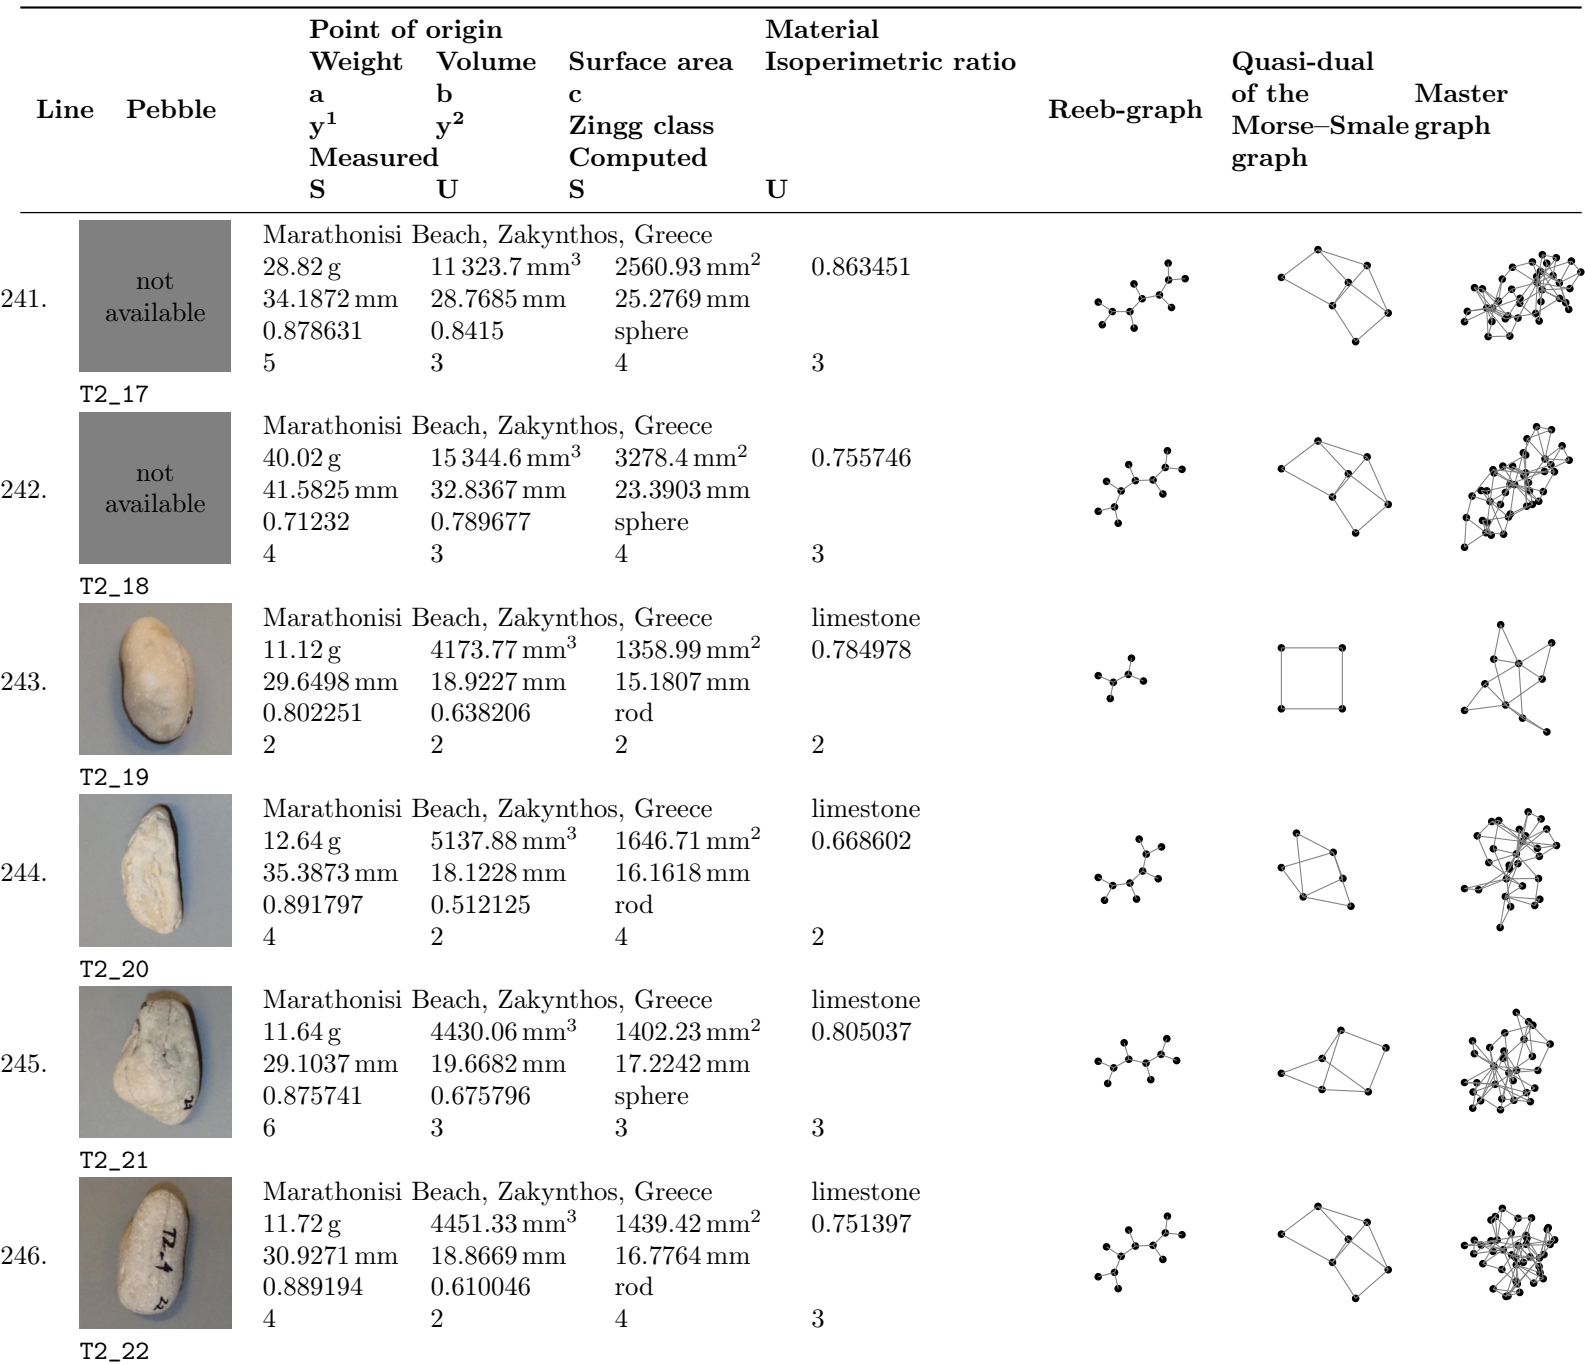   | 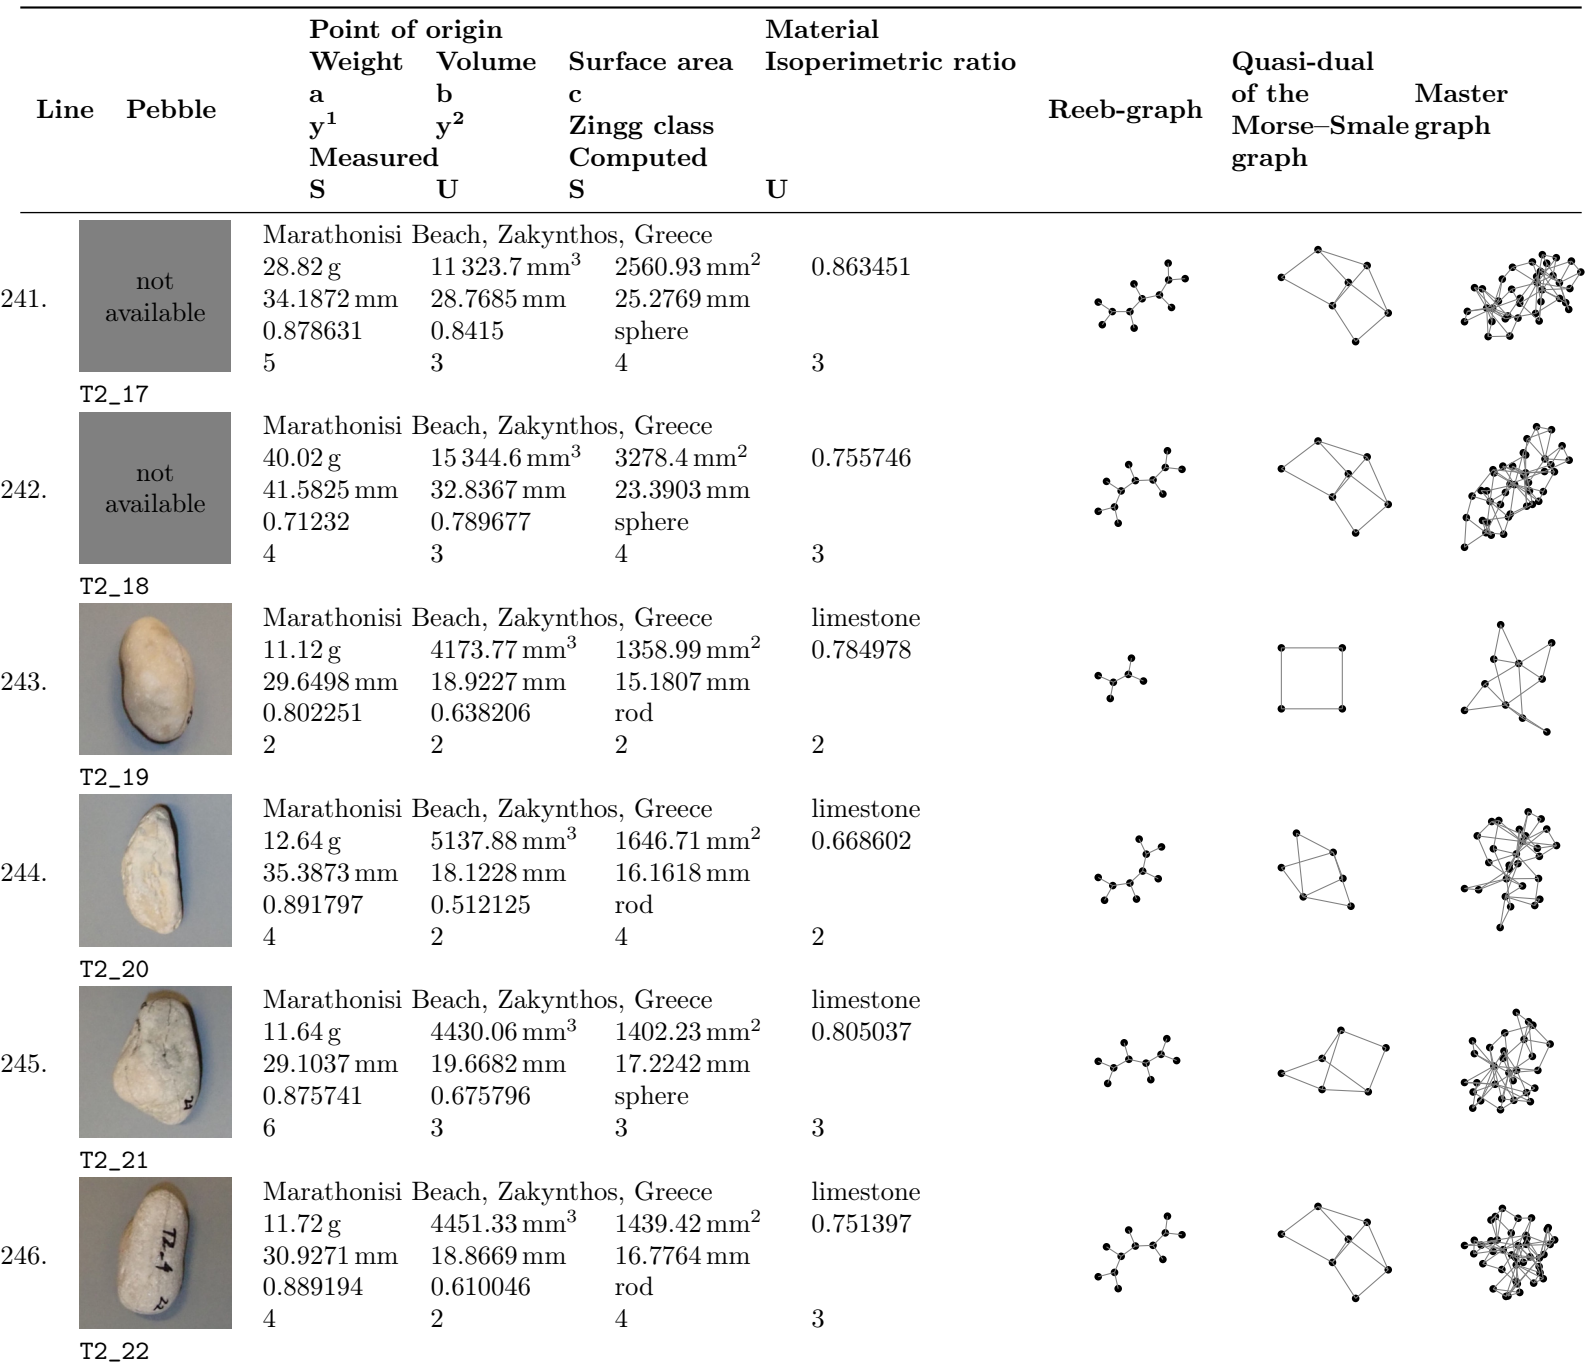   |
|      | T2_17                                                                               |                                                                                |                                                         |                                                      |                                      |                                                                                       |                                                                                       |                                                                                       |
| 242. | 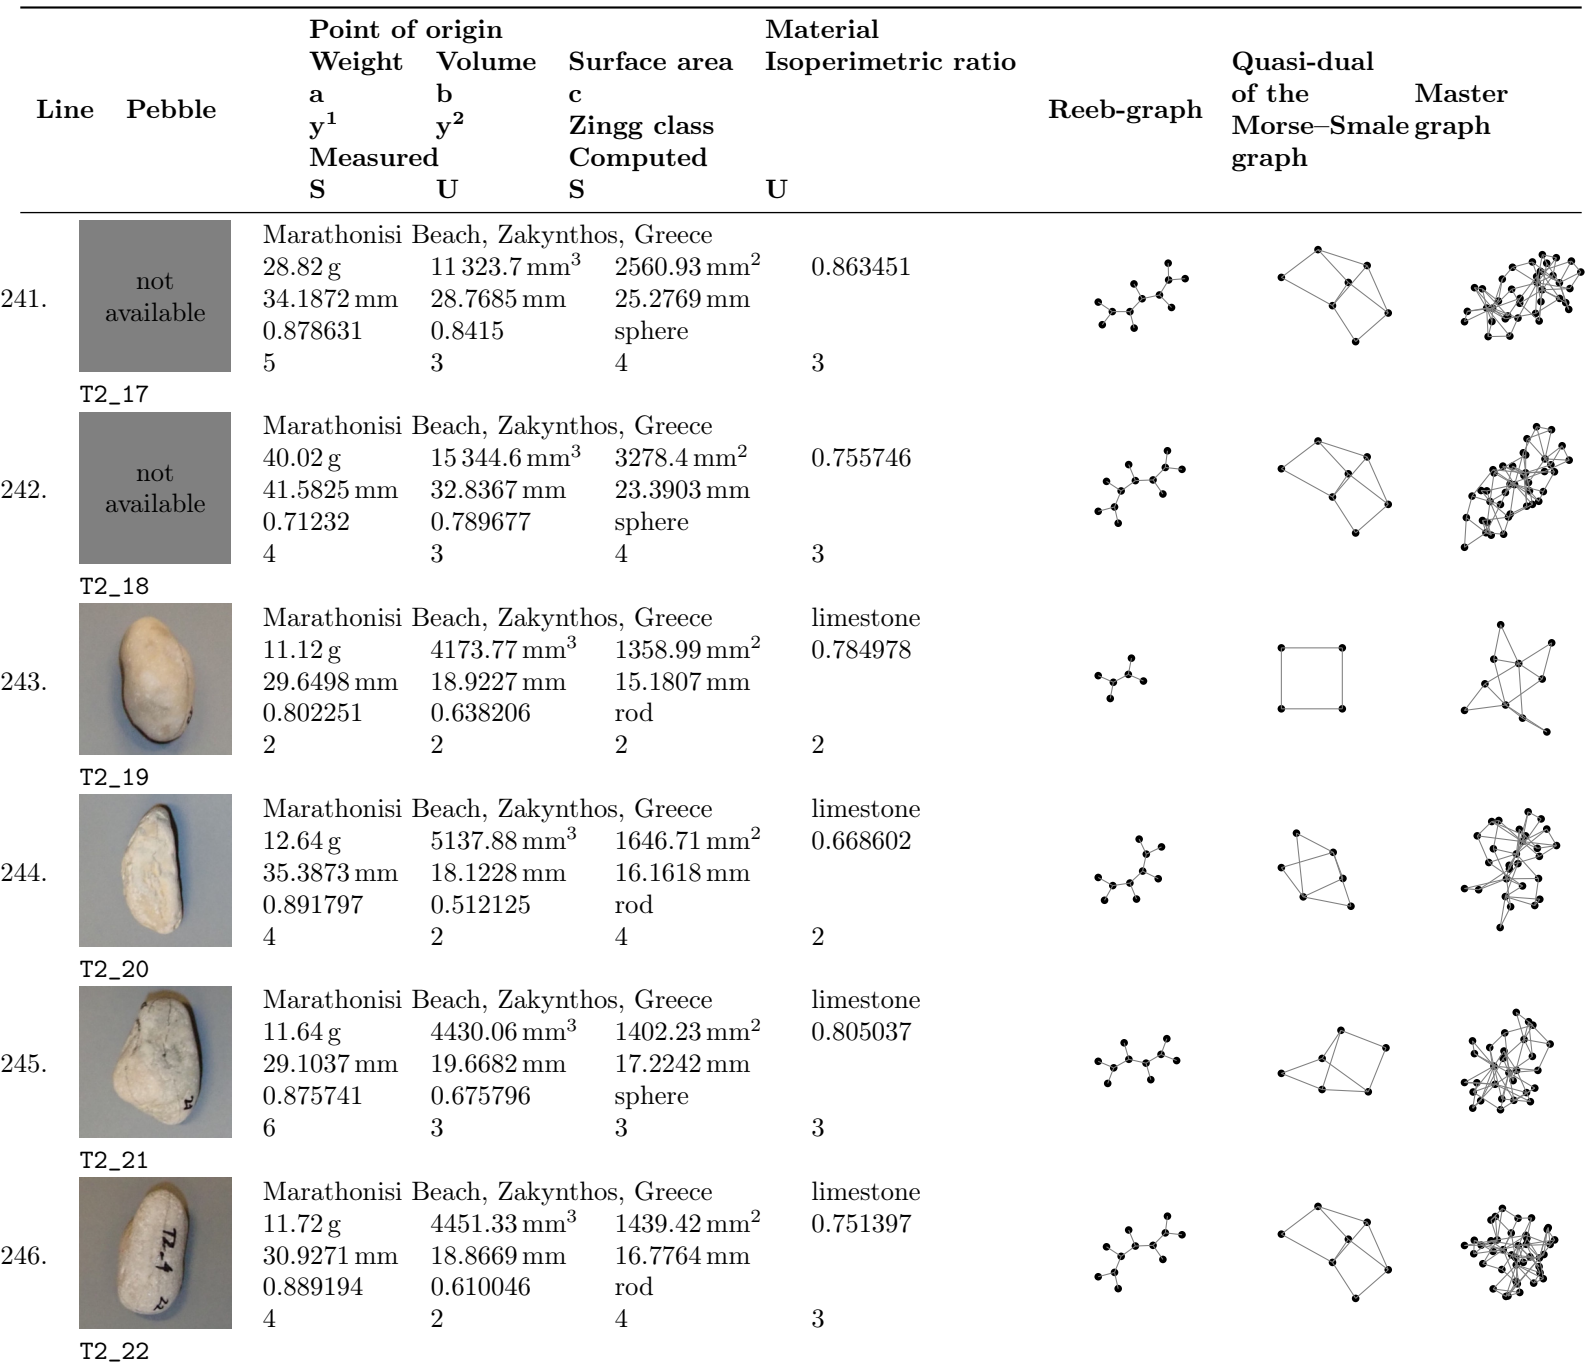   | Marathonisi Beach, Zakynthos, Greece<br>40.02 g<br>41.5825 mm<br>0.71232<br>4  | 15 344.6 mm <sup>3</sup><br>32.8367 mm<br>0.789677<br>3 | 3278.4 mm <sup>2</sup><br>23.3903 mm<br>sphere<br>4  | 0.755746<br><br><br>3                | 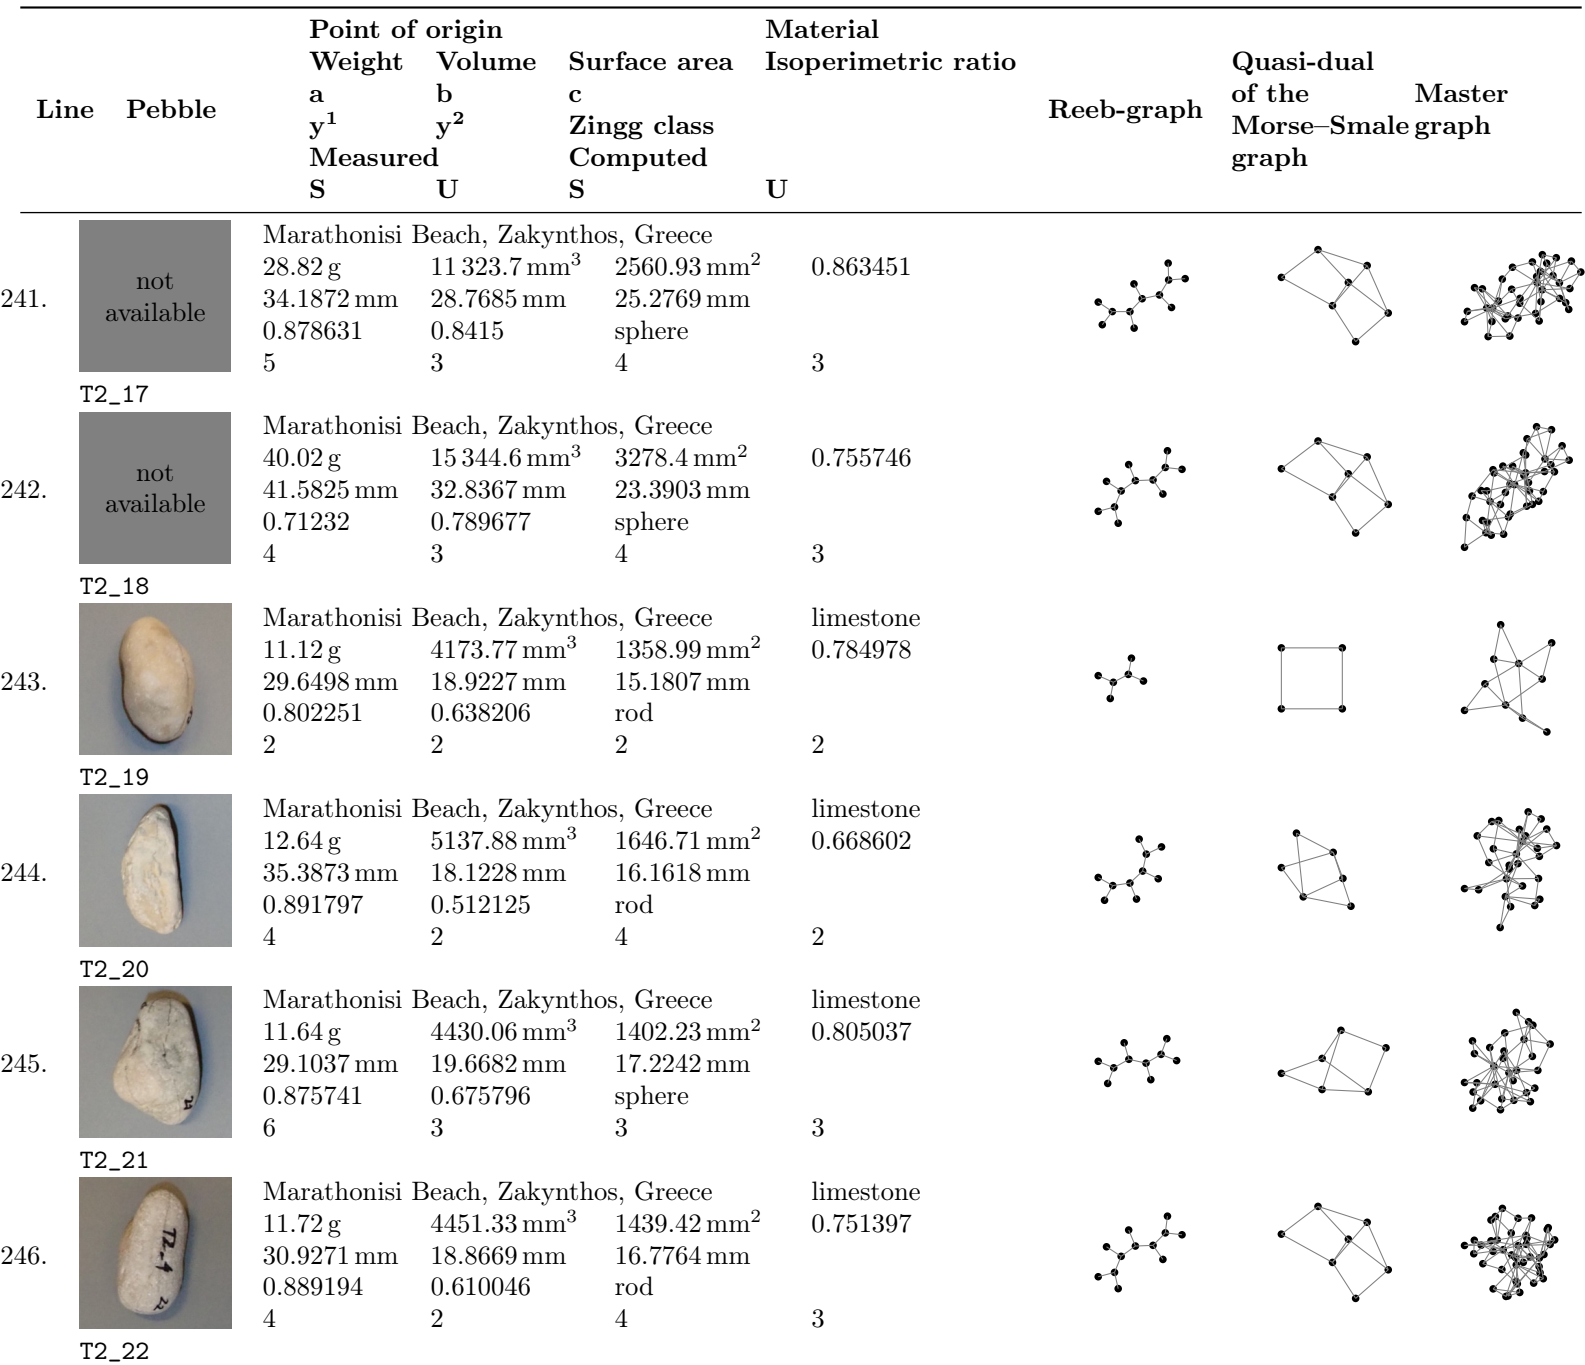   | 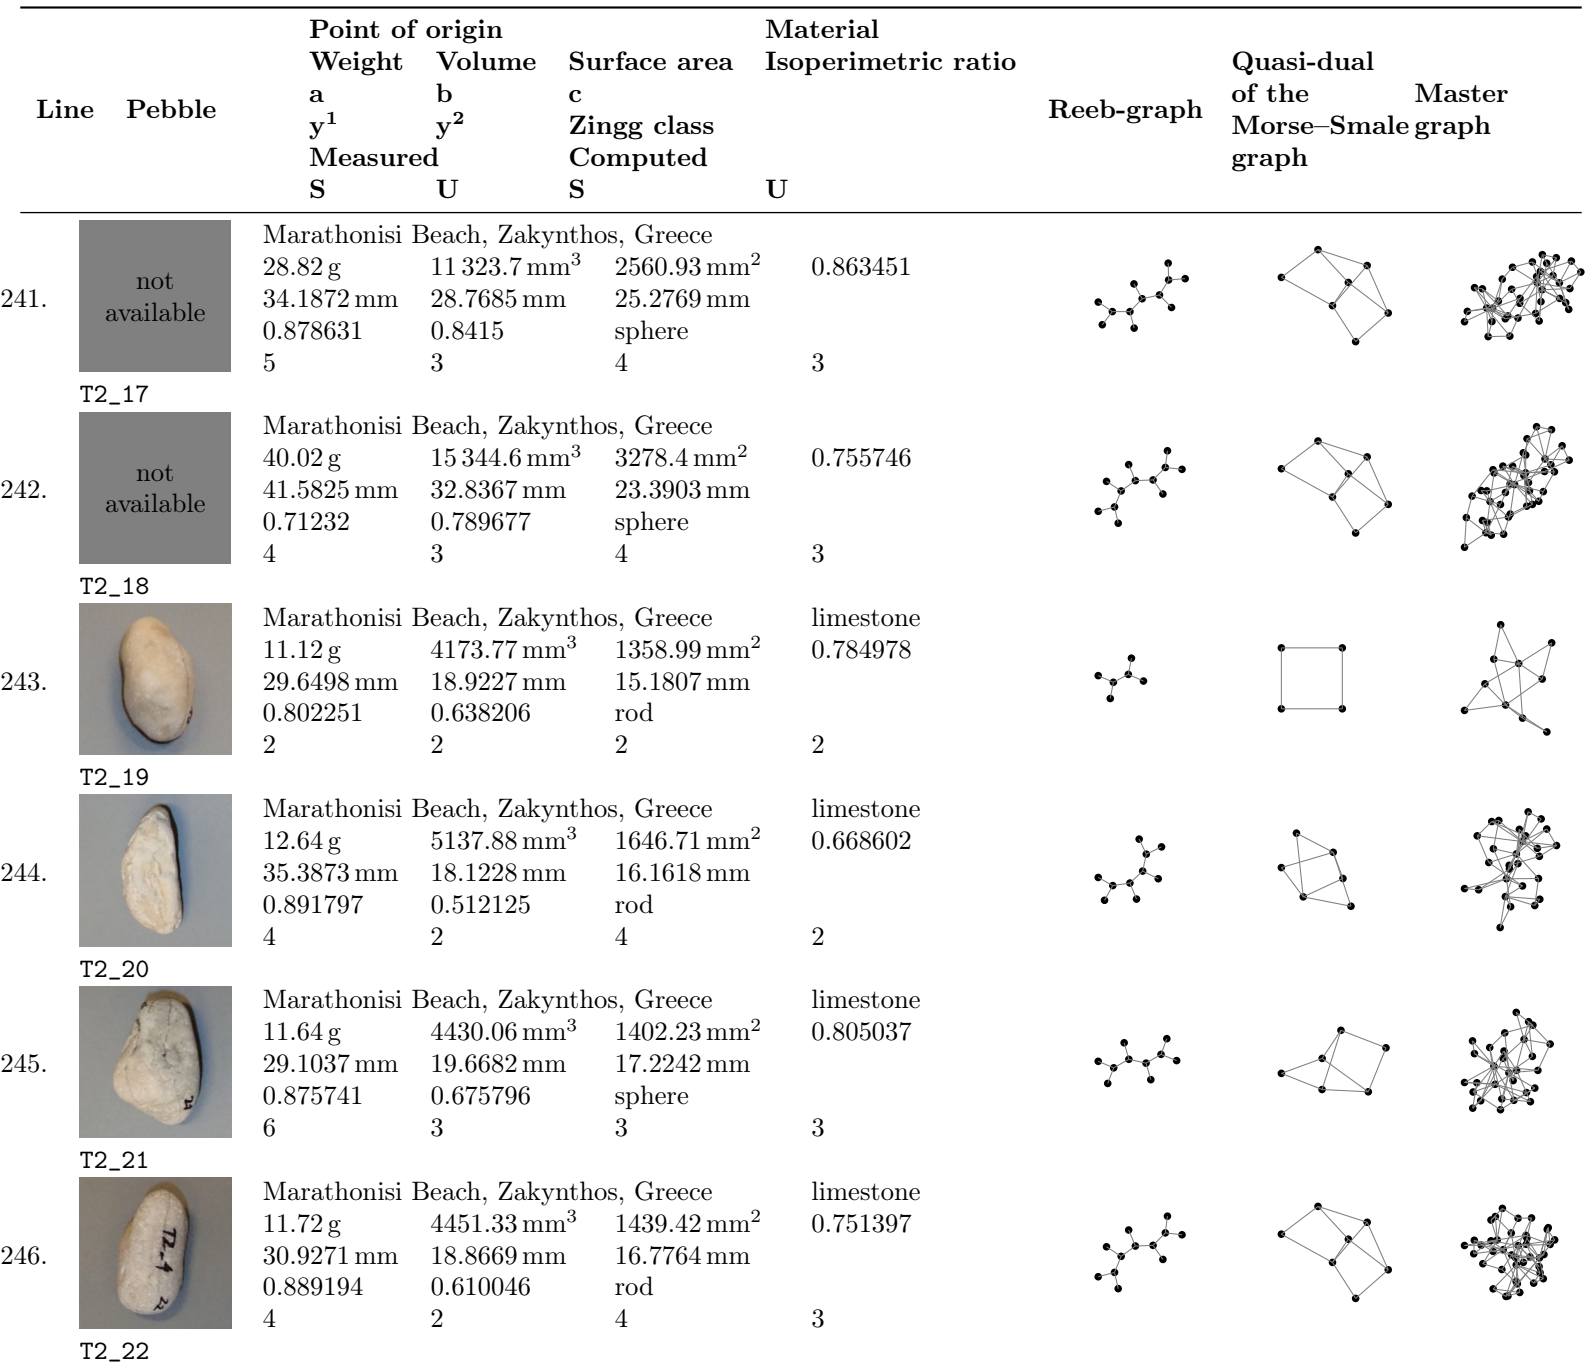   | 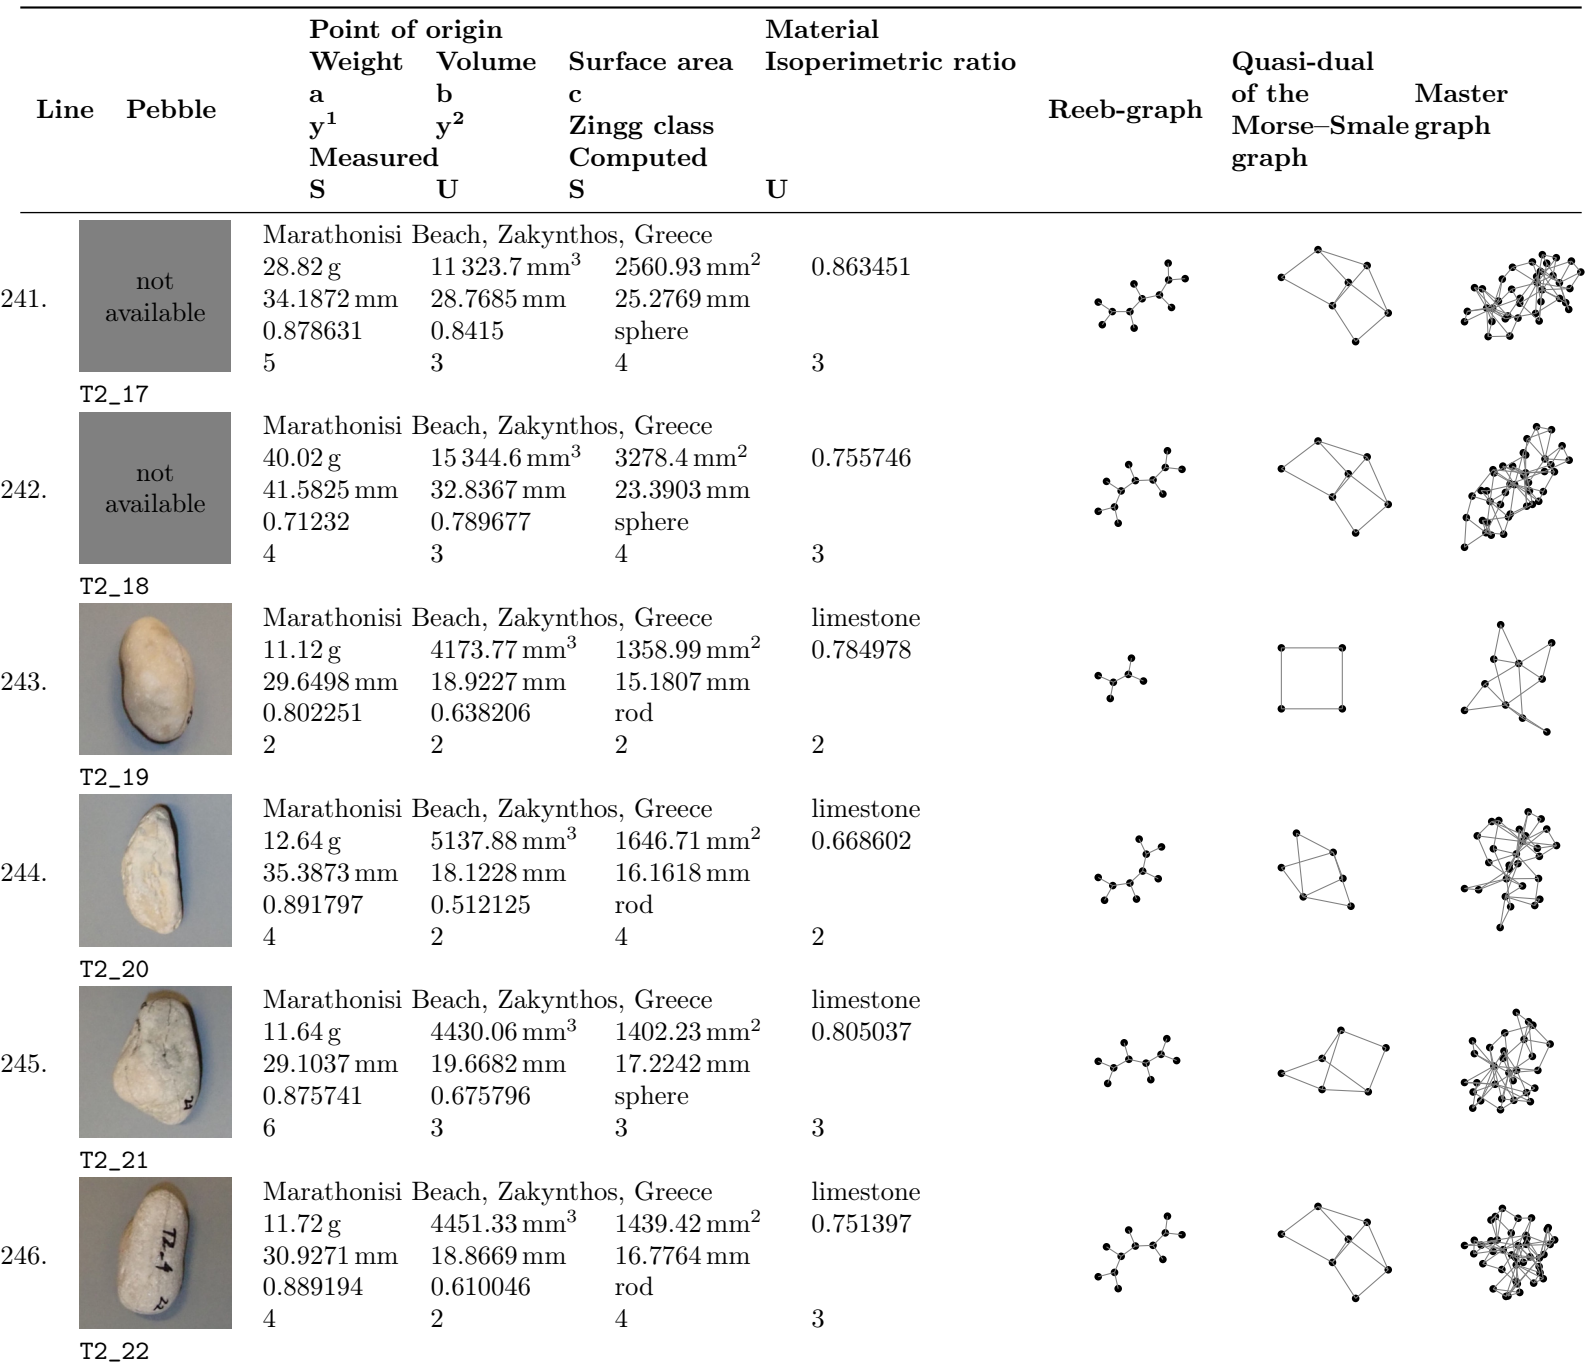   |
|      | T2_18                                                                               |                                                                                |                                                         |                                                      |                                      |                                                                                       |                                                                                       |                                                                                       |
| 243. | 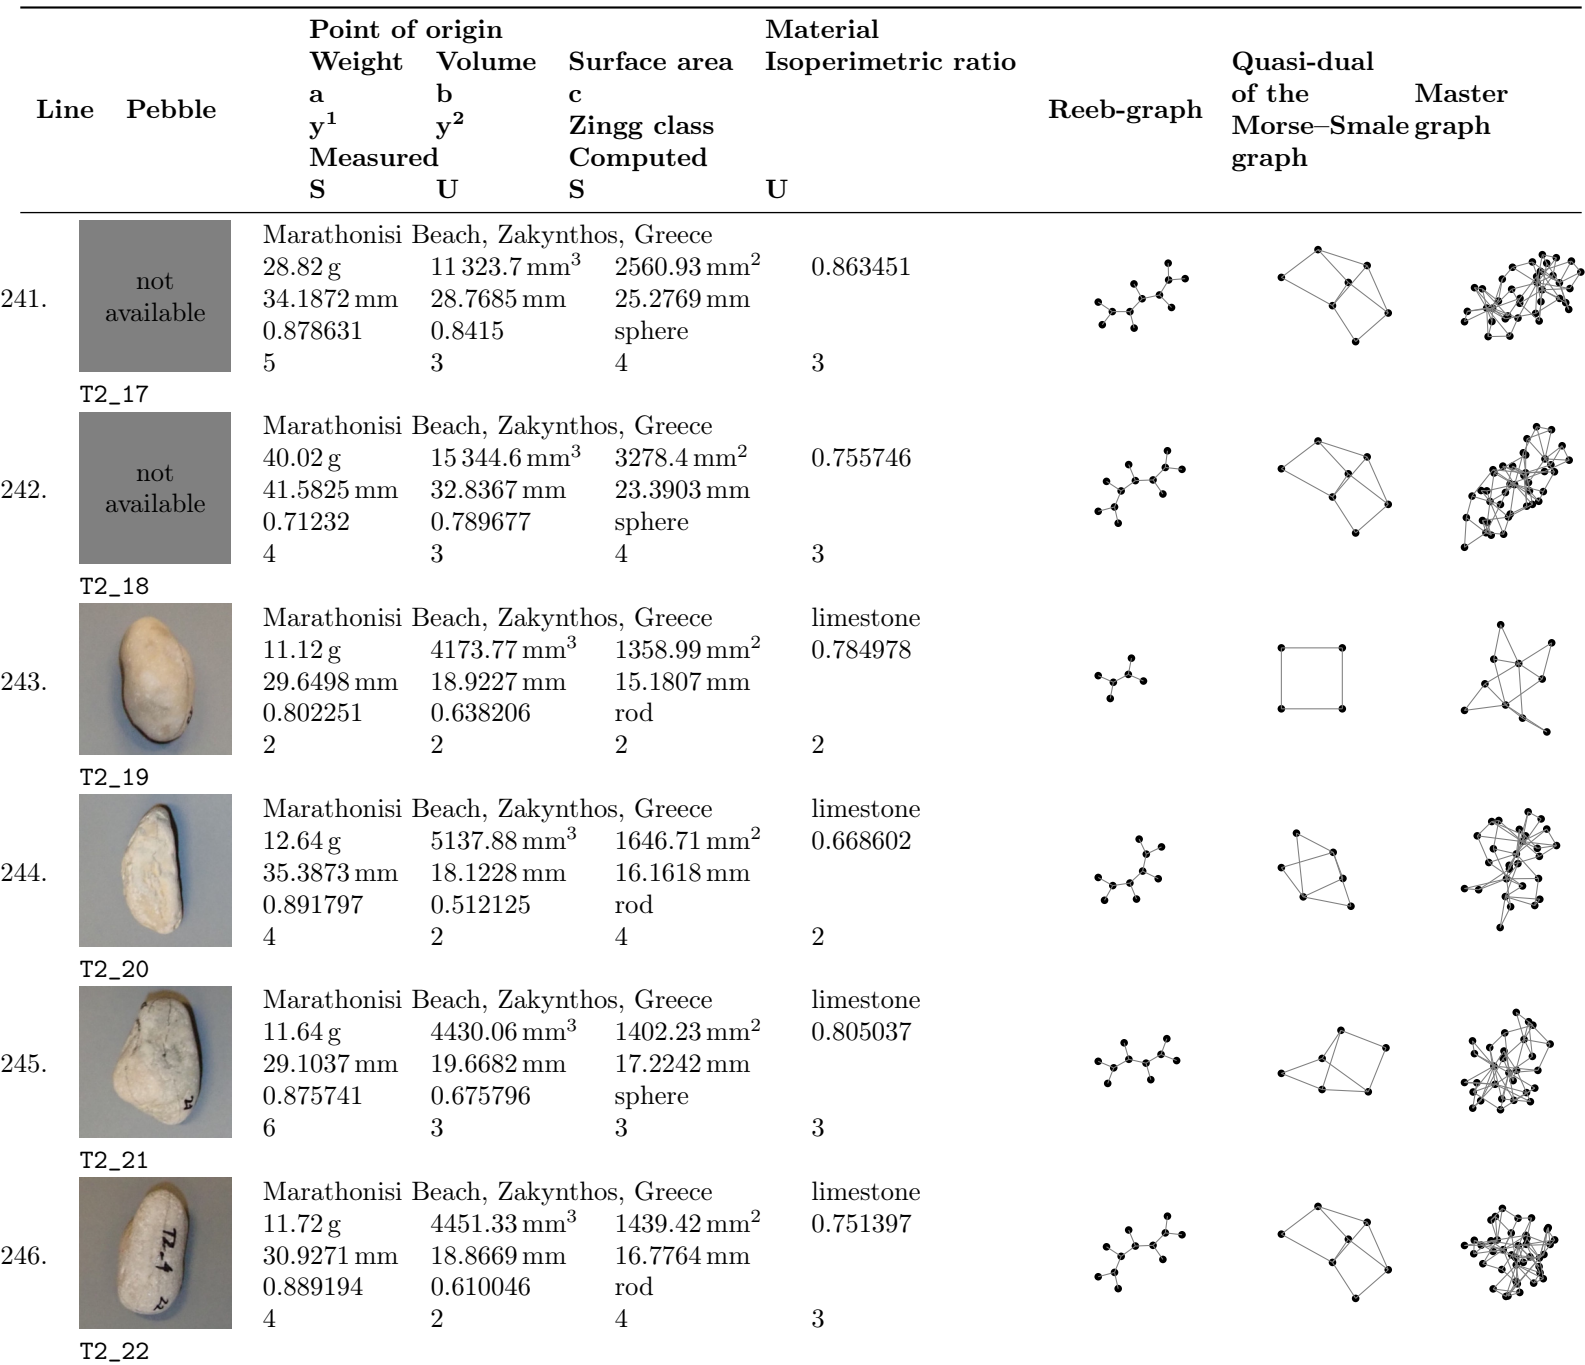   | Marathonisi Beach, Zakynthos, Greece<br>11.12 g<br>29.6498 mm<br>0.802251<br>2 | 4173.77 mm <sup>3</sup><br>18.9227 mm<br>0.638206<br>2  | 1358.99 mm <sup>2</sup><br>15.1807 mm<br>rod<br>2    | limestone<br>0.784978<br><br>2       | 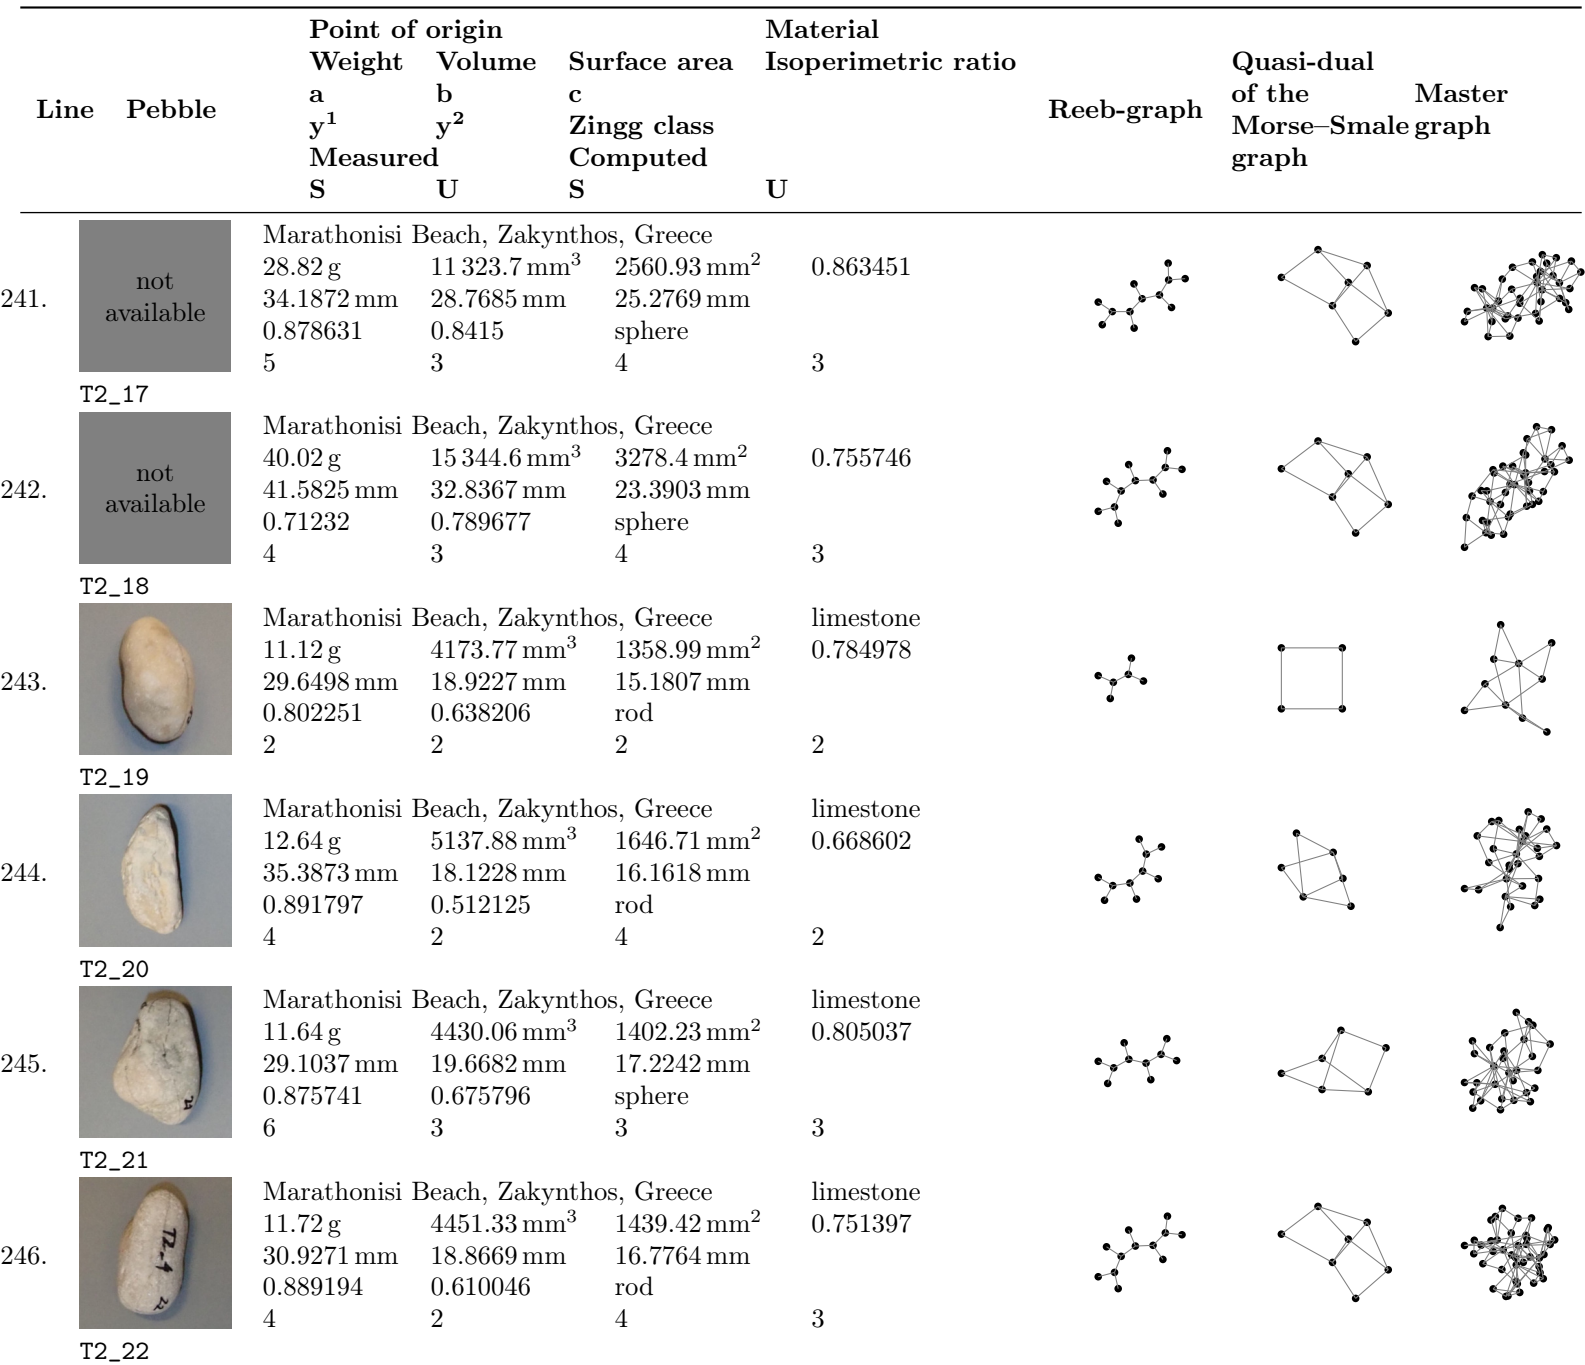   | 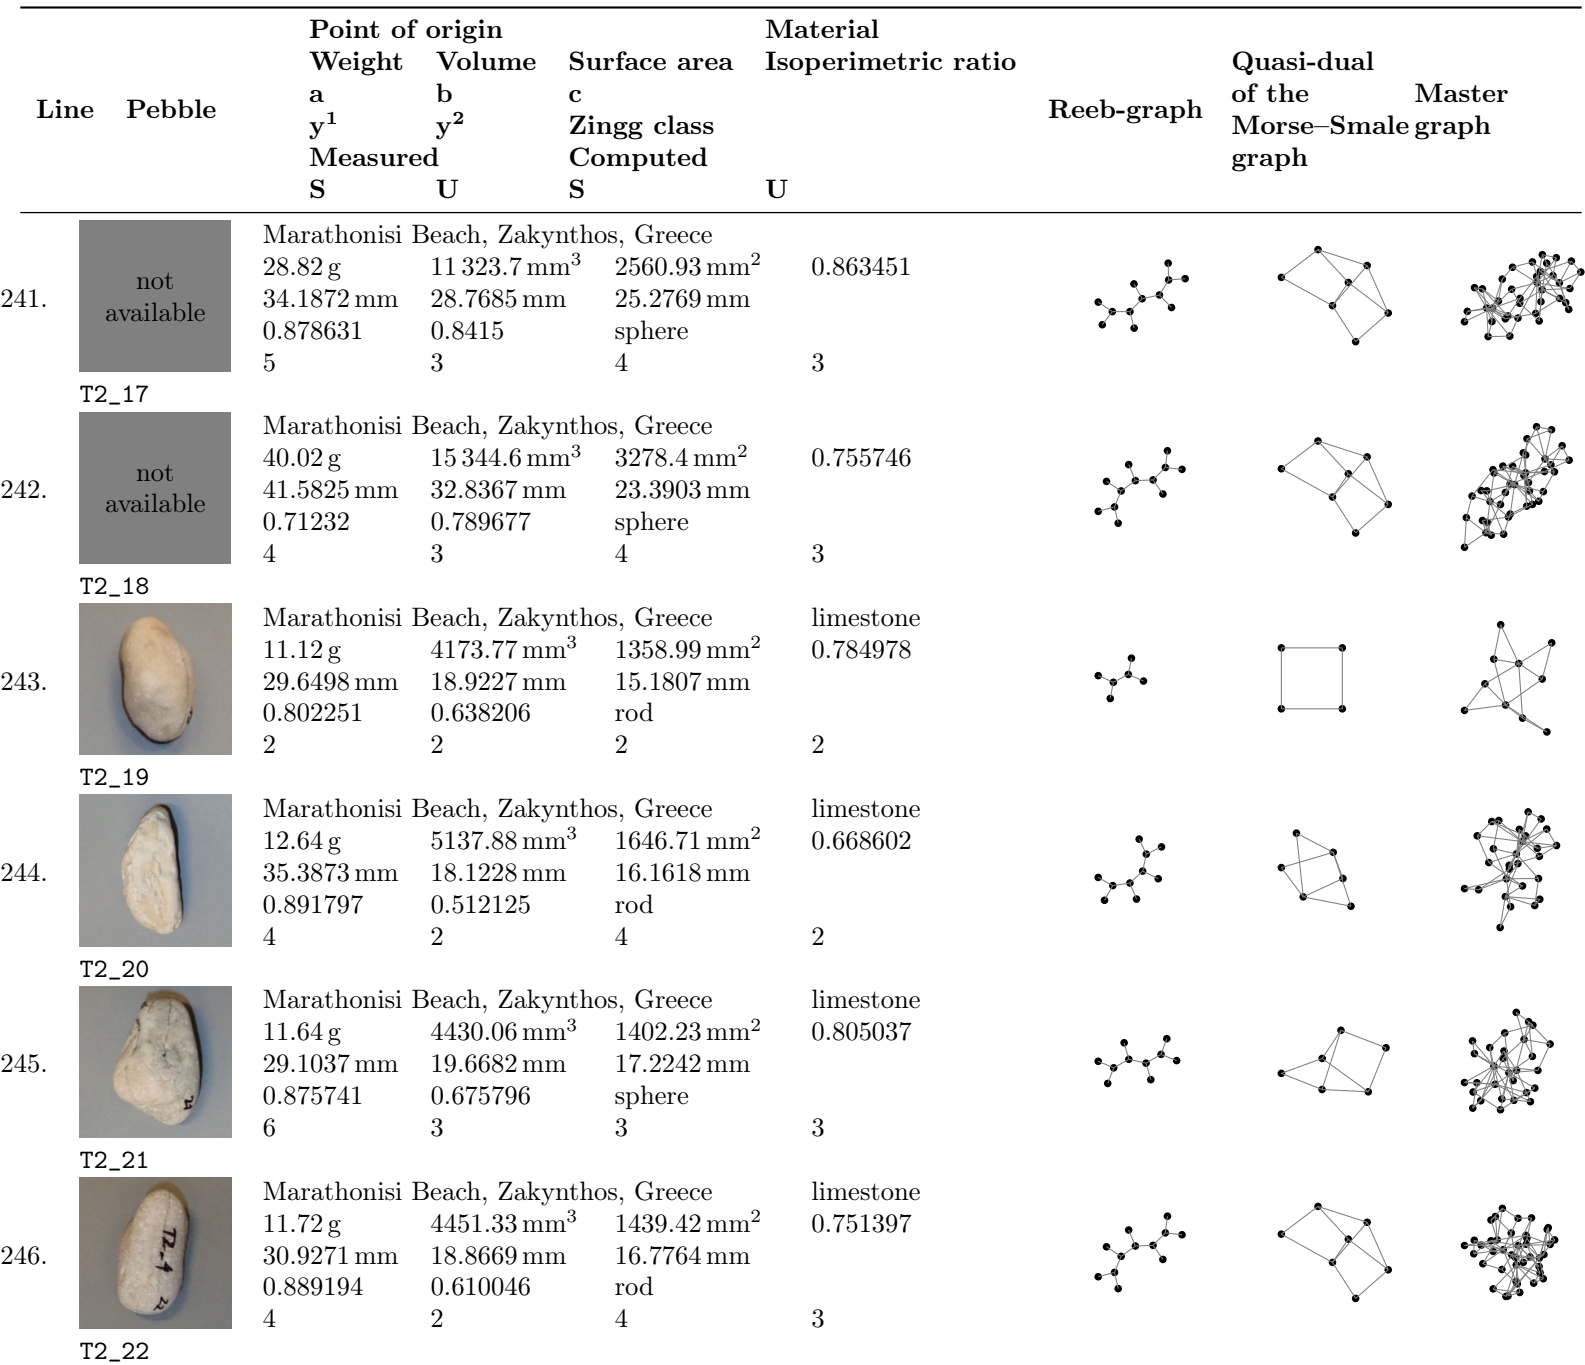   | 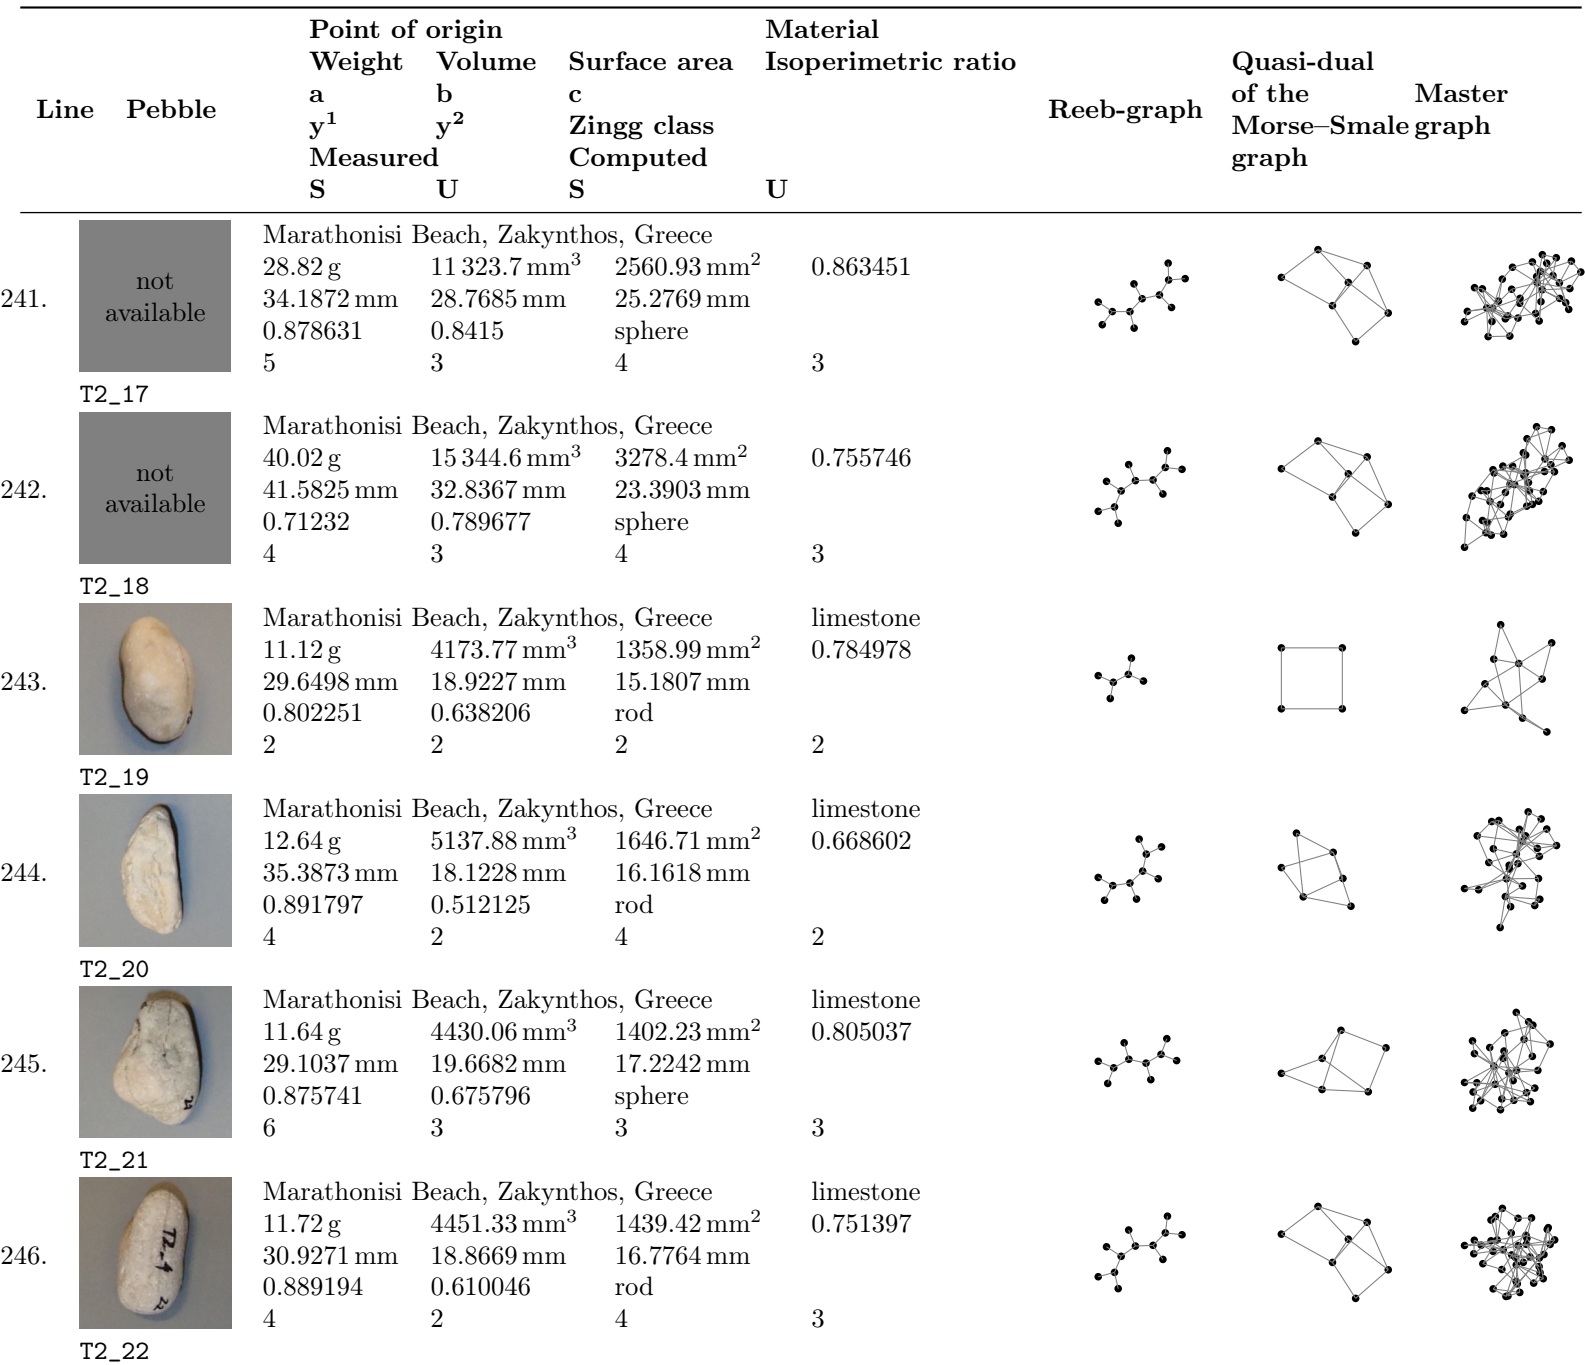   |
|      | T2_19                                                                               |                                                                                |                                                         |                                                      |                                      |                                                                                       |                                                                                       |                                                                                       |
| 244. | 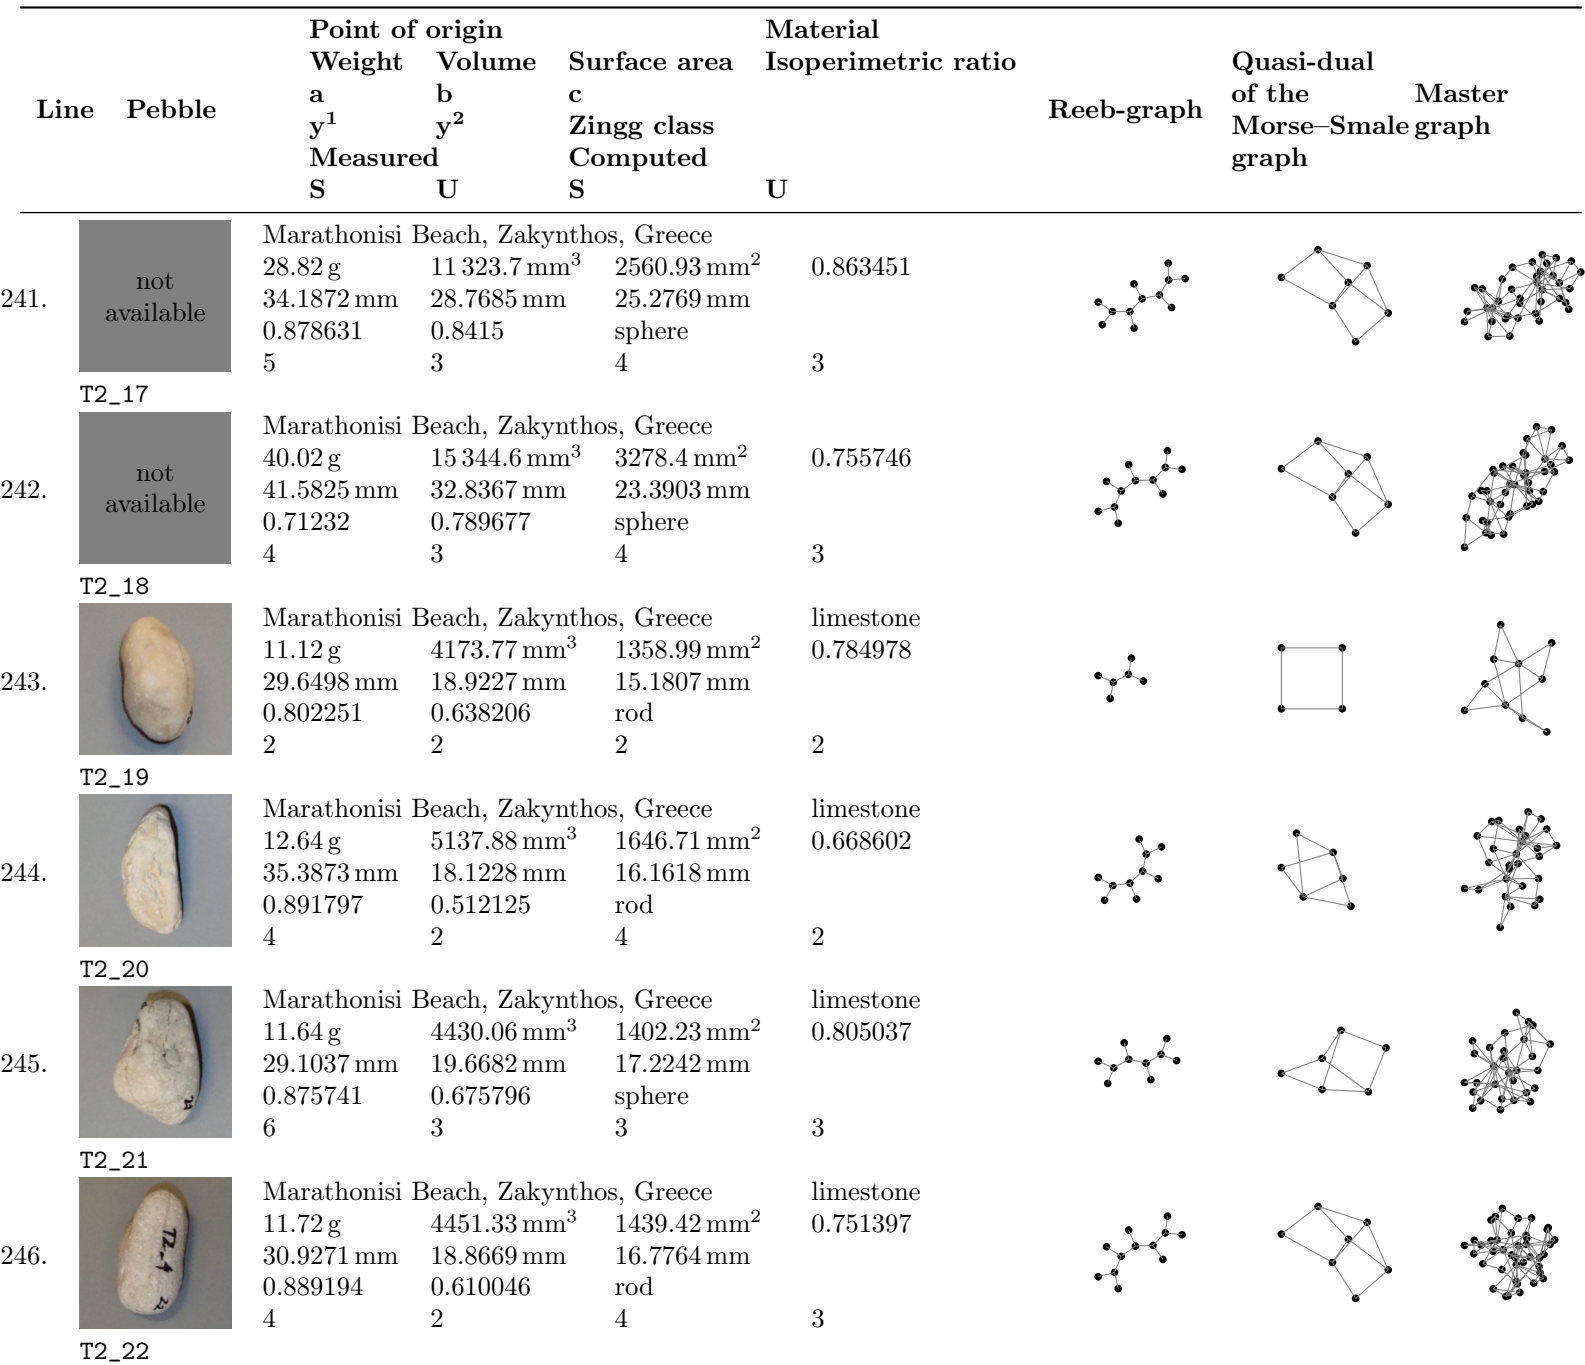  | Marathonisi Beach, Zakynthos, Greece<br>12.64 g<br>35.3873 mm<br>0.891797<br>4 | 5137.88 mm <sup>3</sup><br>18.1228 mm<br>0.512125<br>2  | 1646.71 mm <sup>2</sup><br>16.1618 mm<br>rod<br>4    | limestone<br>0.668602<br><br>2       | 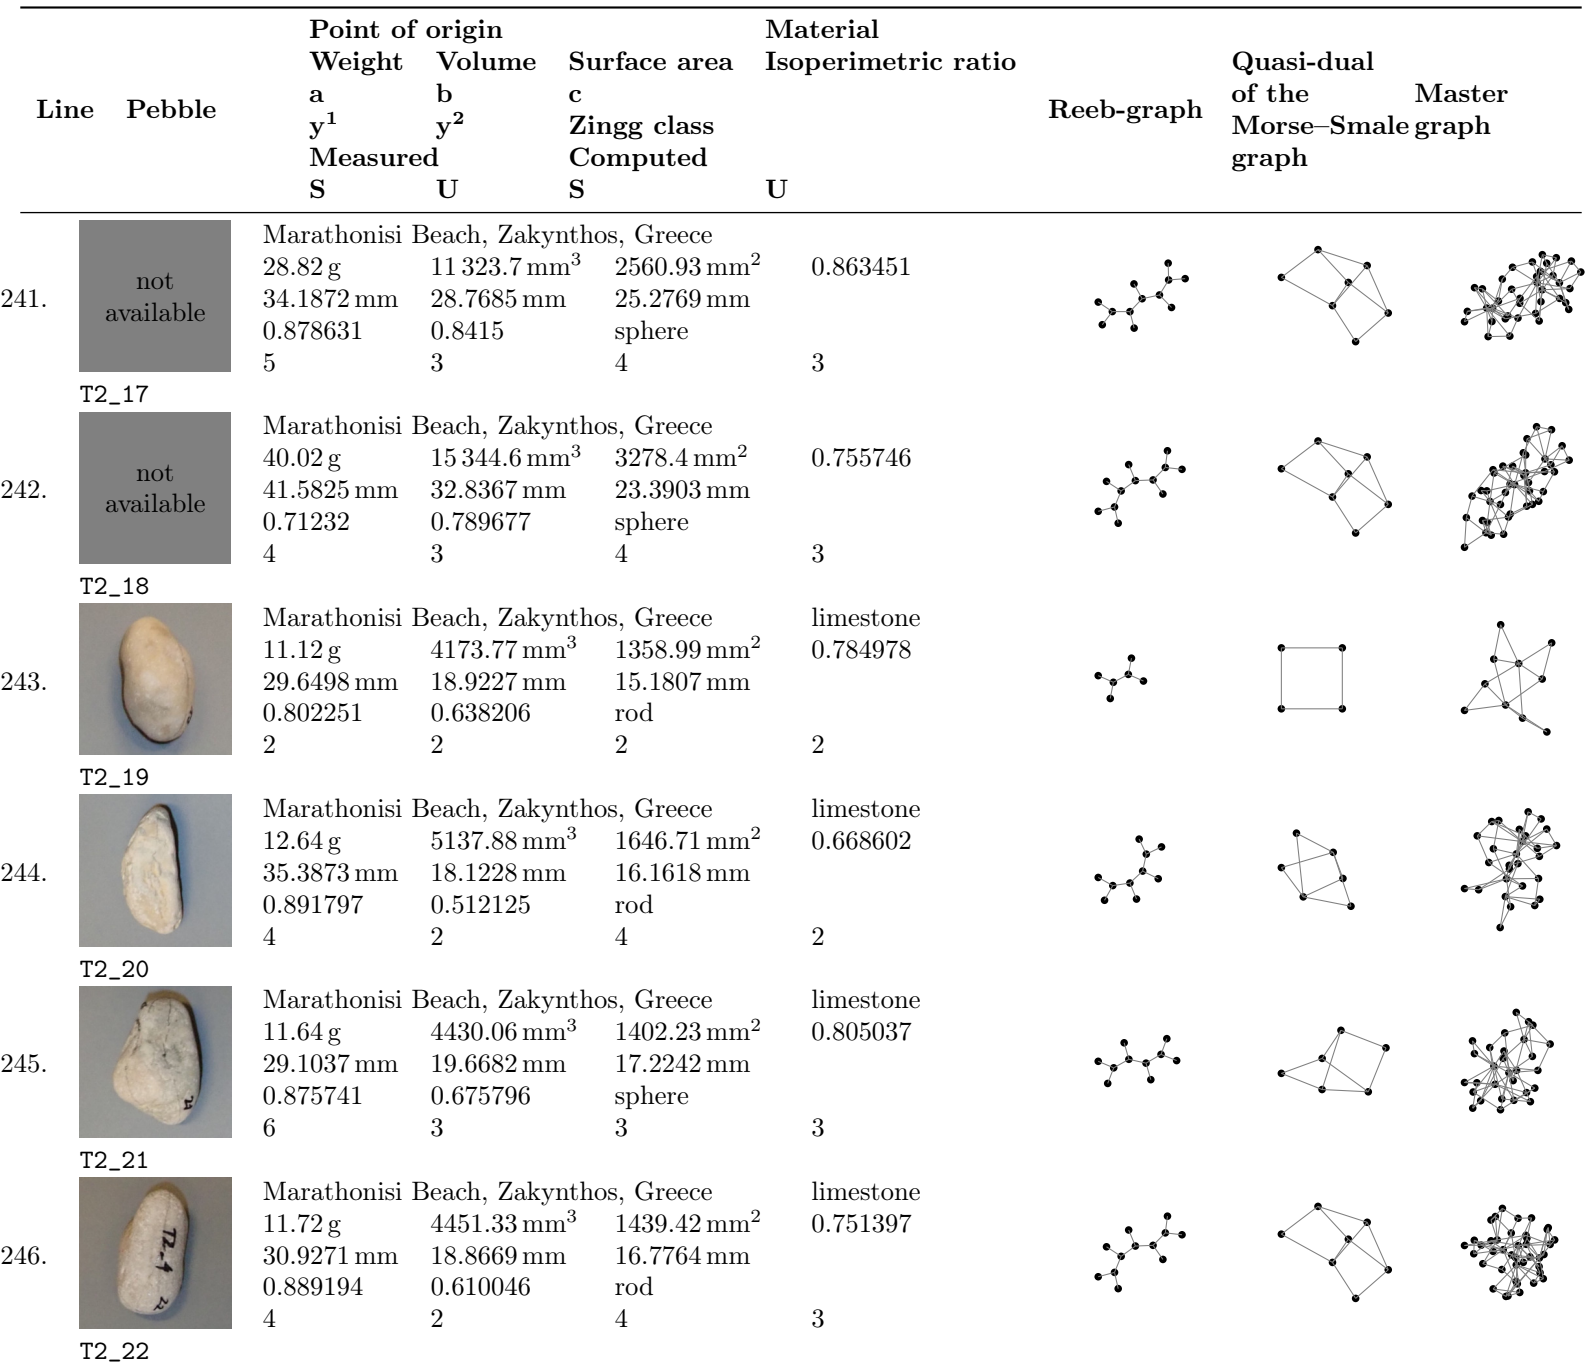  | 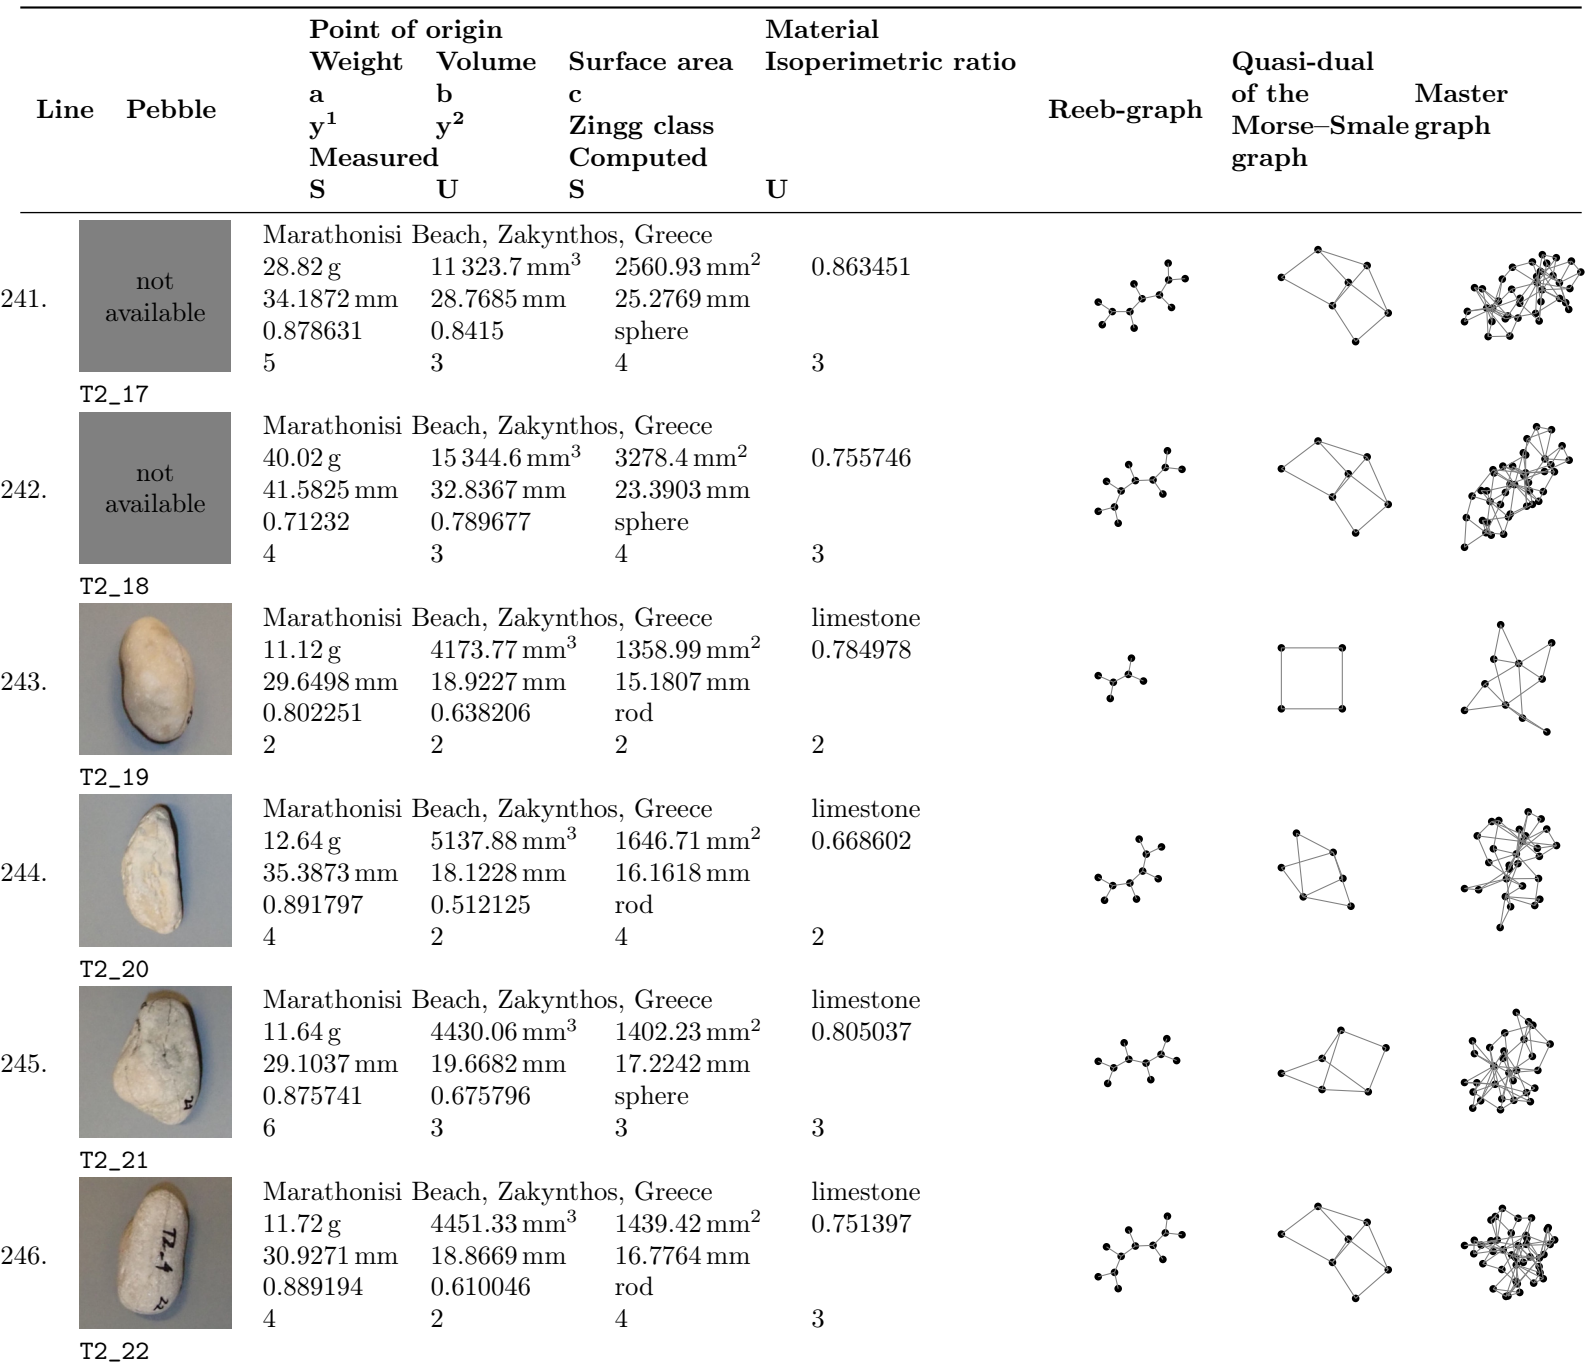  | 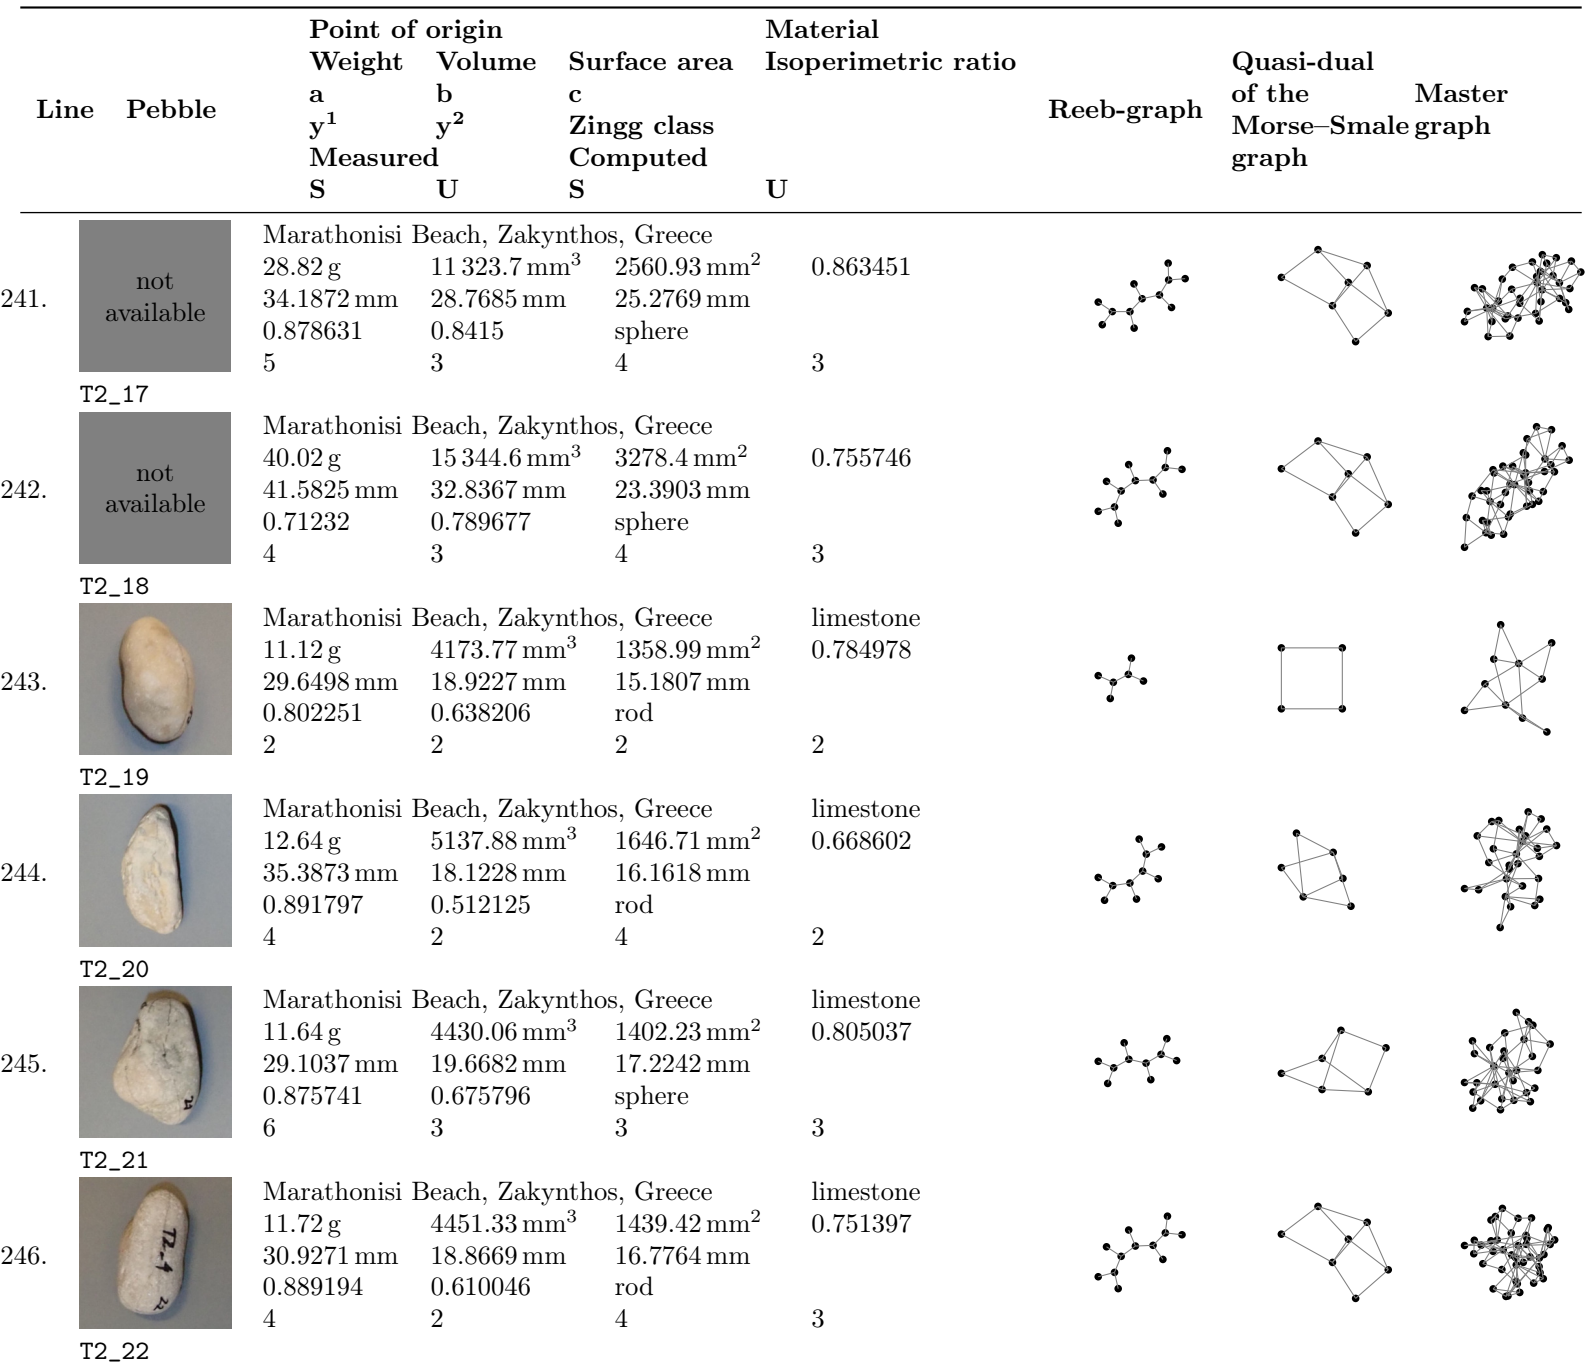  |
|      | T2_20                                                                               |                                                                                |                                                         |                                                      |                                      |                                                                                       |                                                                                       |                                                                                       |
| 245. | 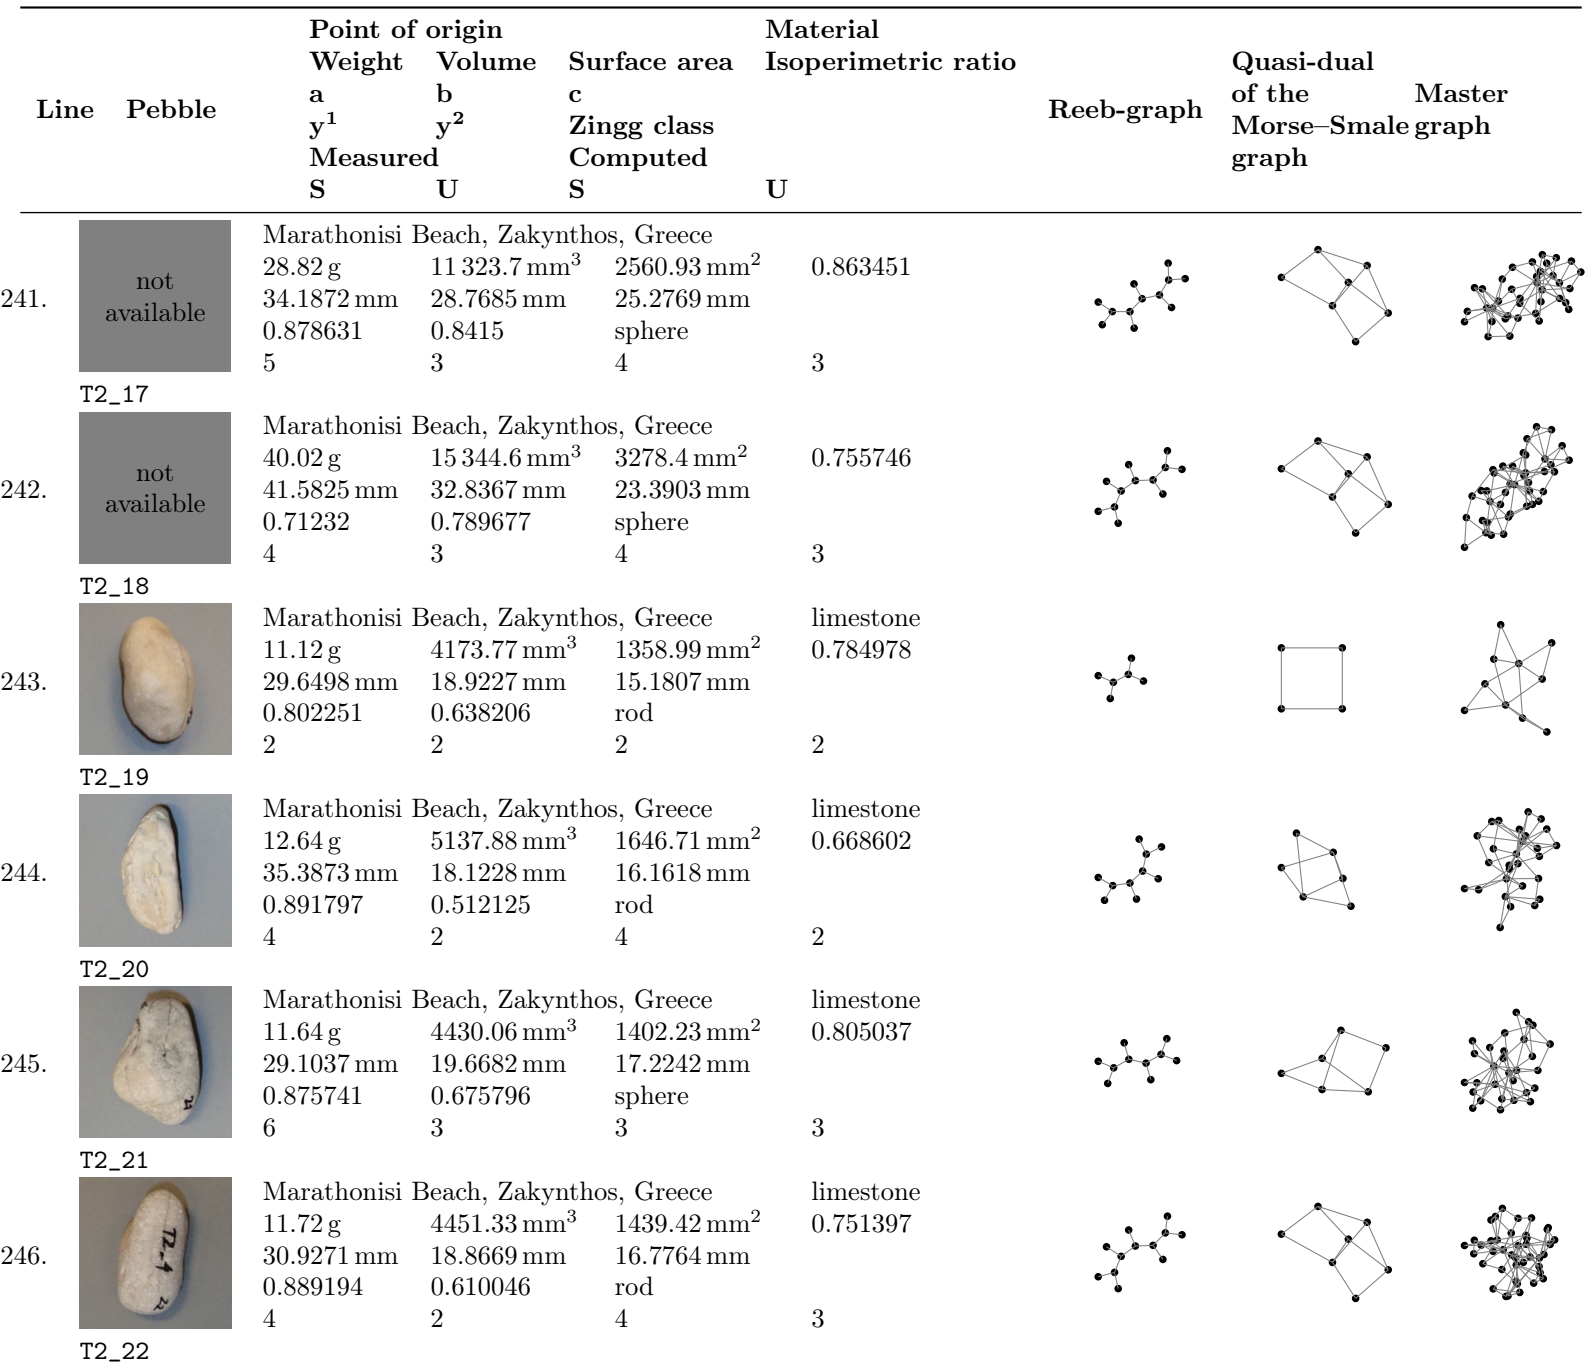 | Marathonisi Beach, Zakynthos, Greece<br>11.64 g<br>29.1037 mm<br>0.875741<br>6 | 4430.06 mm <sup>3</sup><br>19.6682 mm<br>0.675796<br>3  | 1402.23 mm <sup>2</sup><br>17.2242 mm<br>sphere<br>3 | limestone<br>0.805037<br><br>3       | 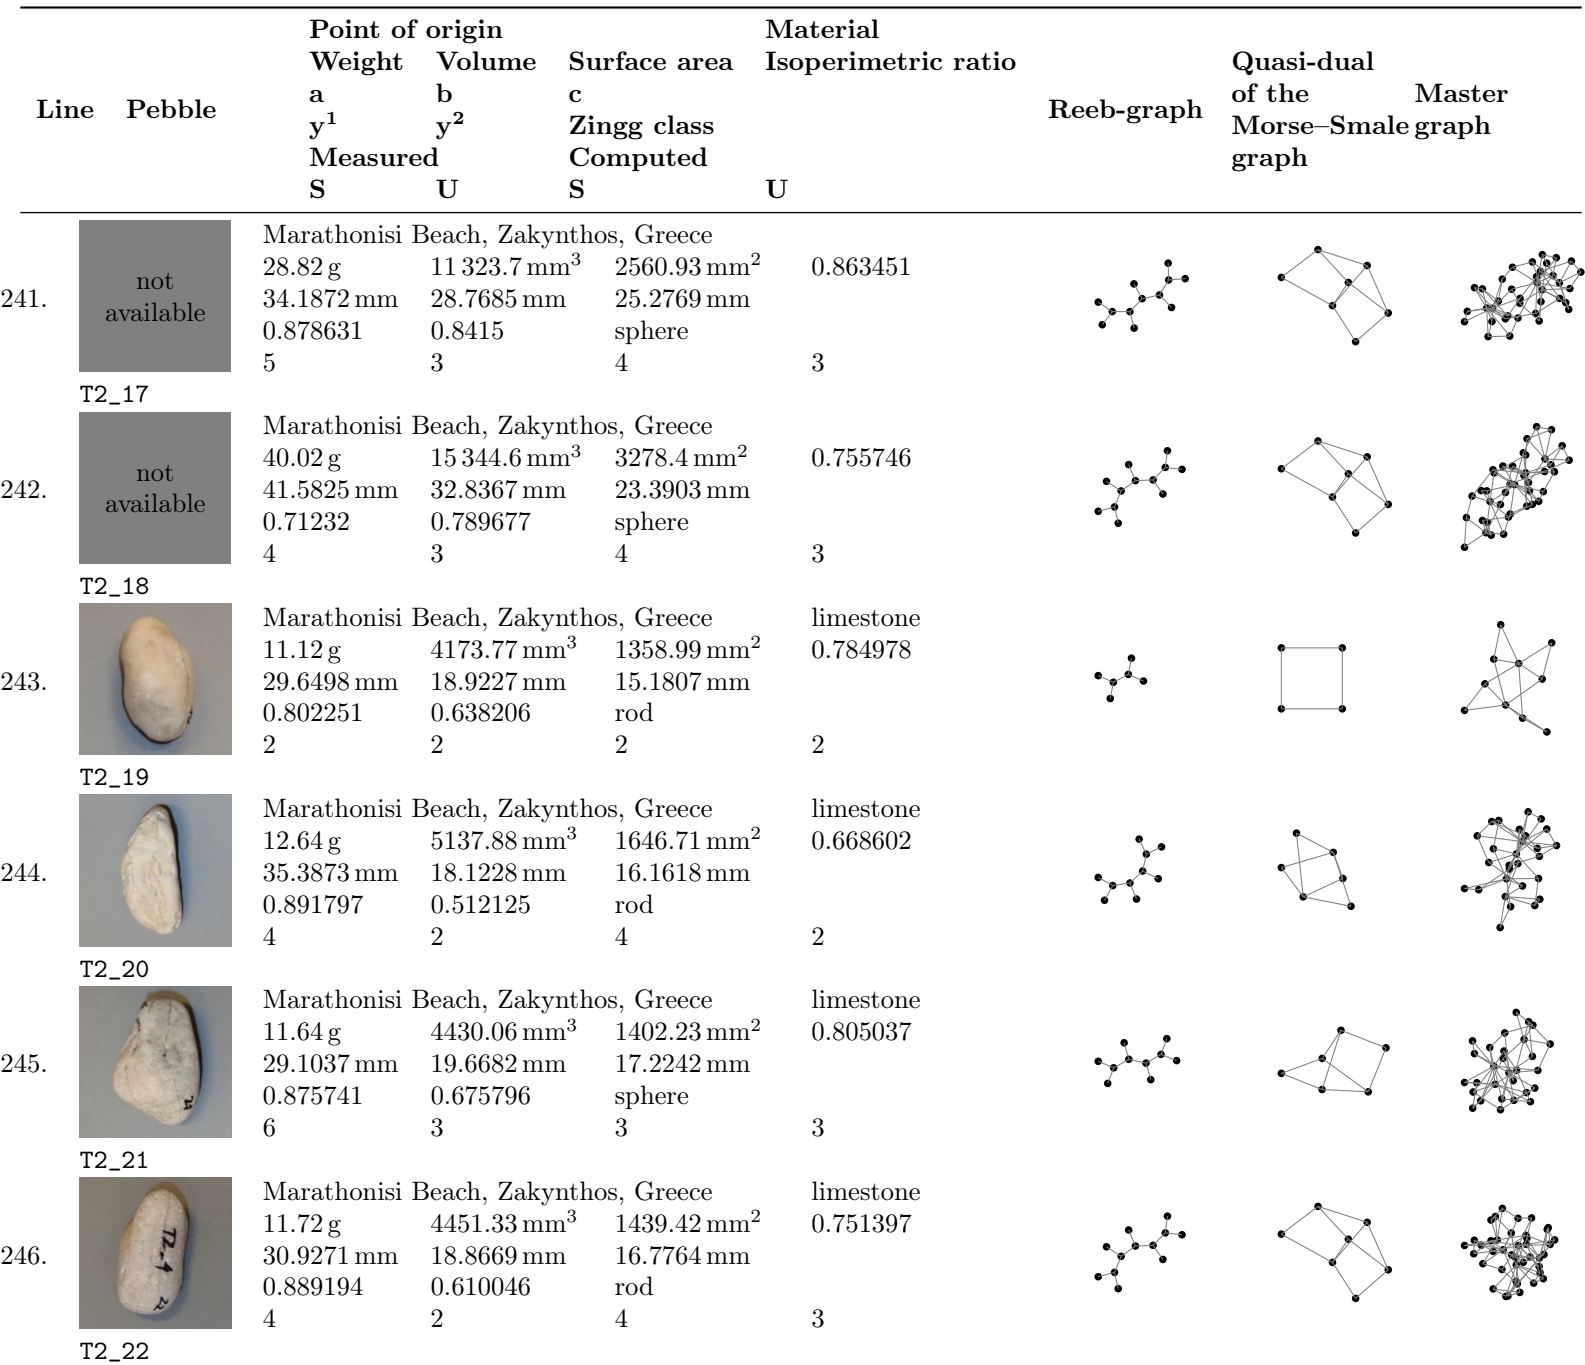 | 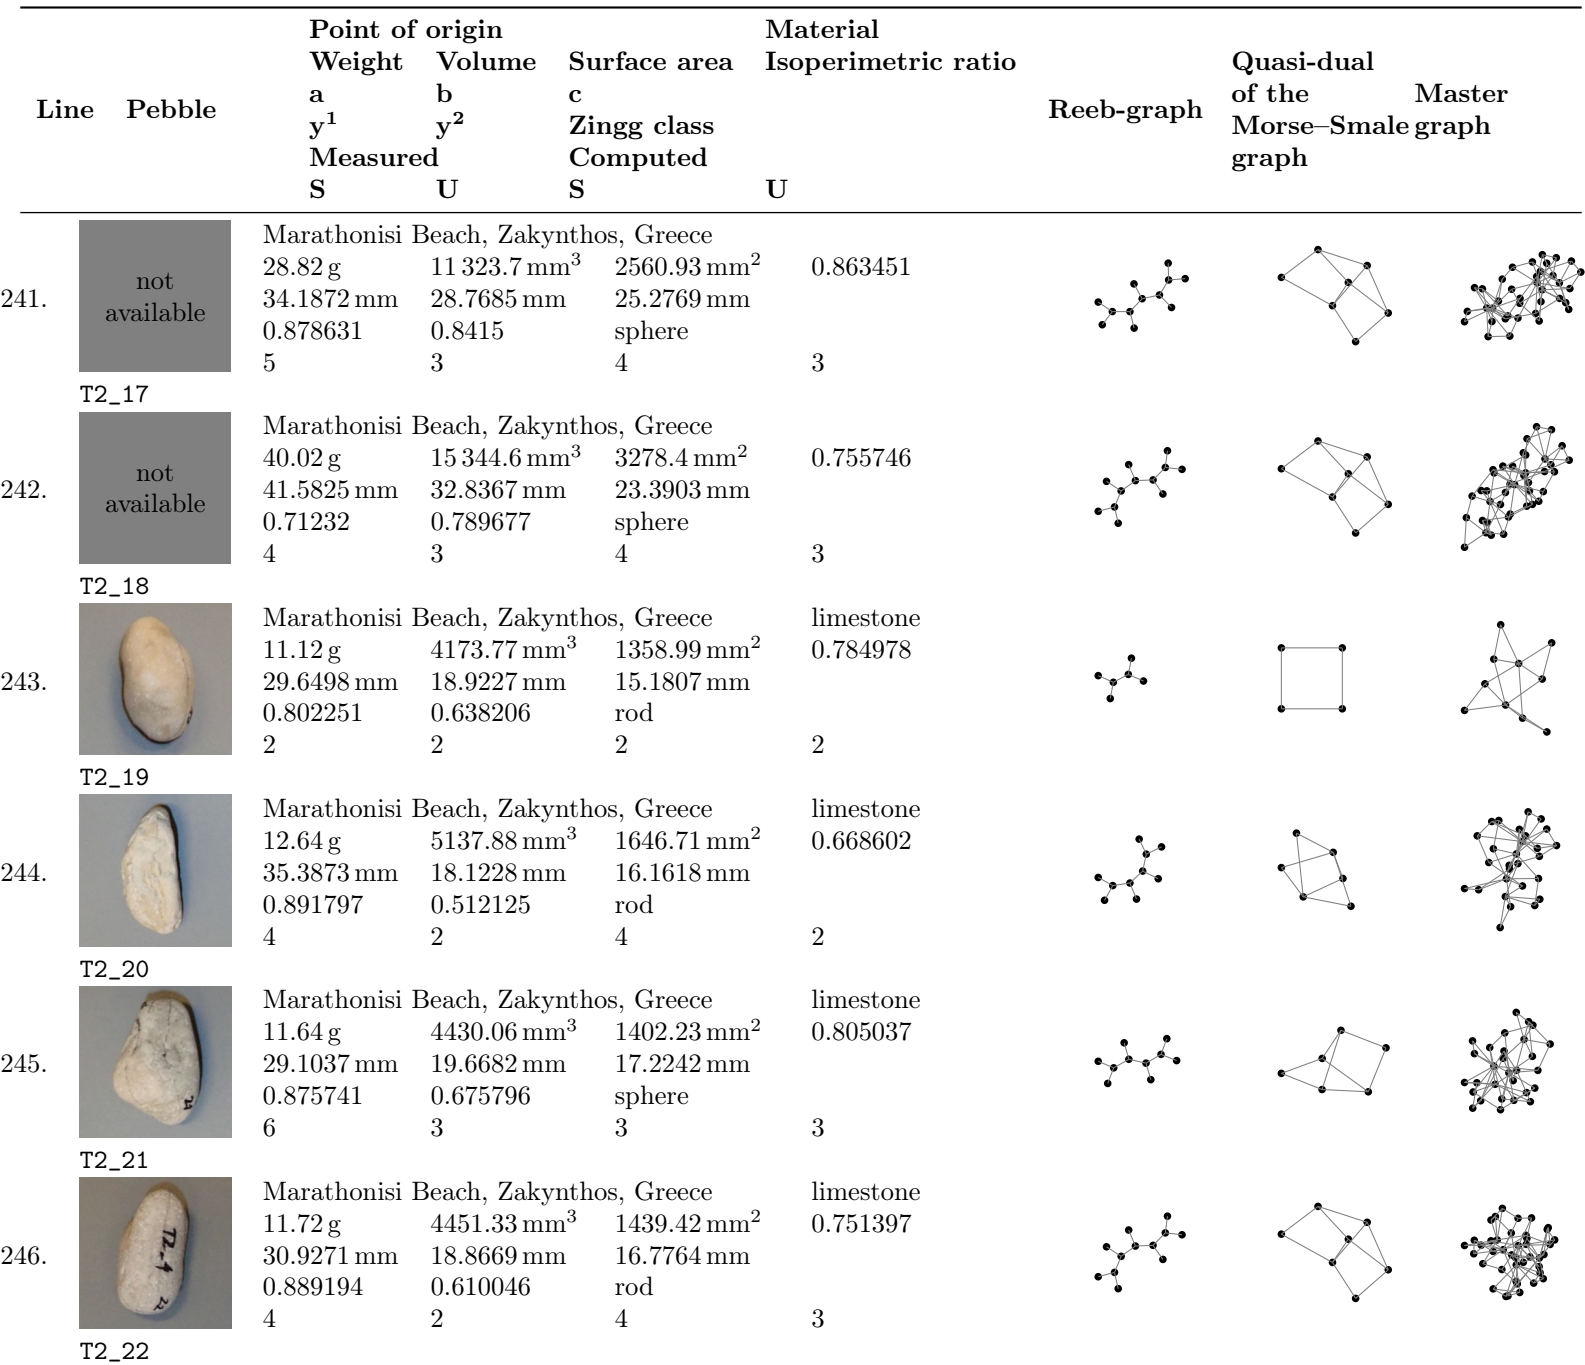 | 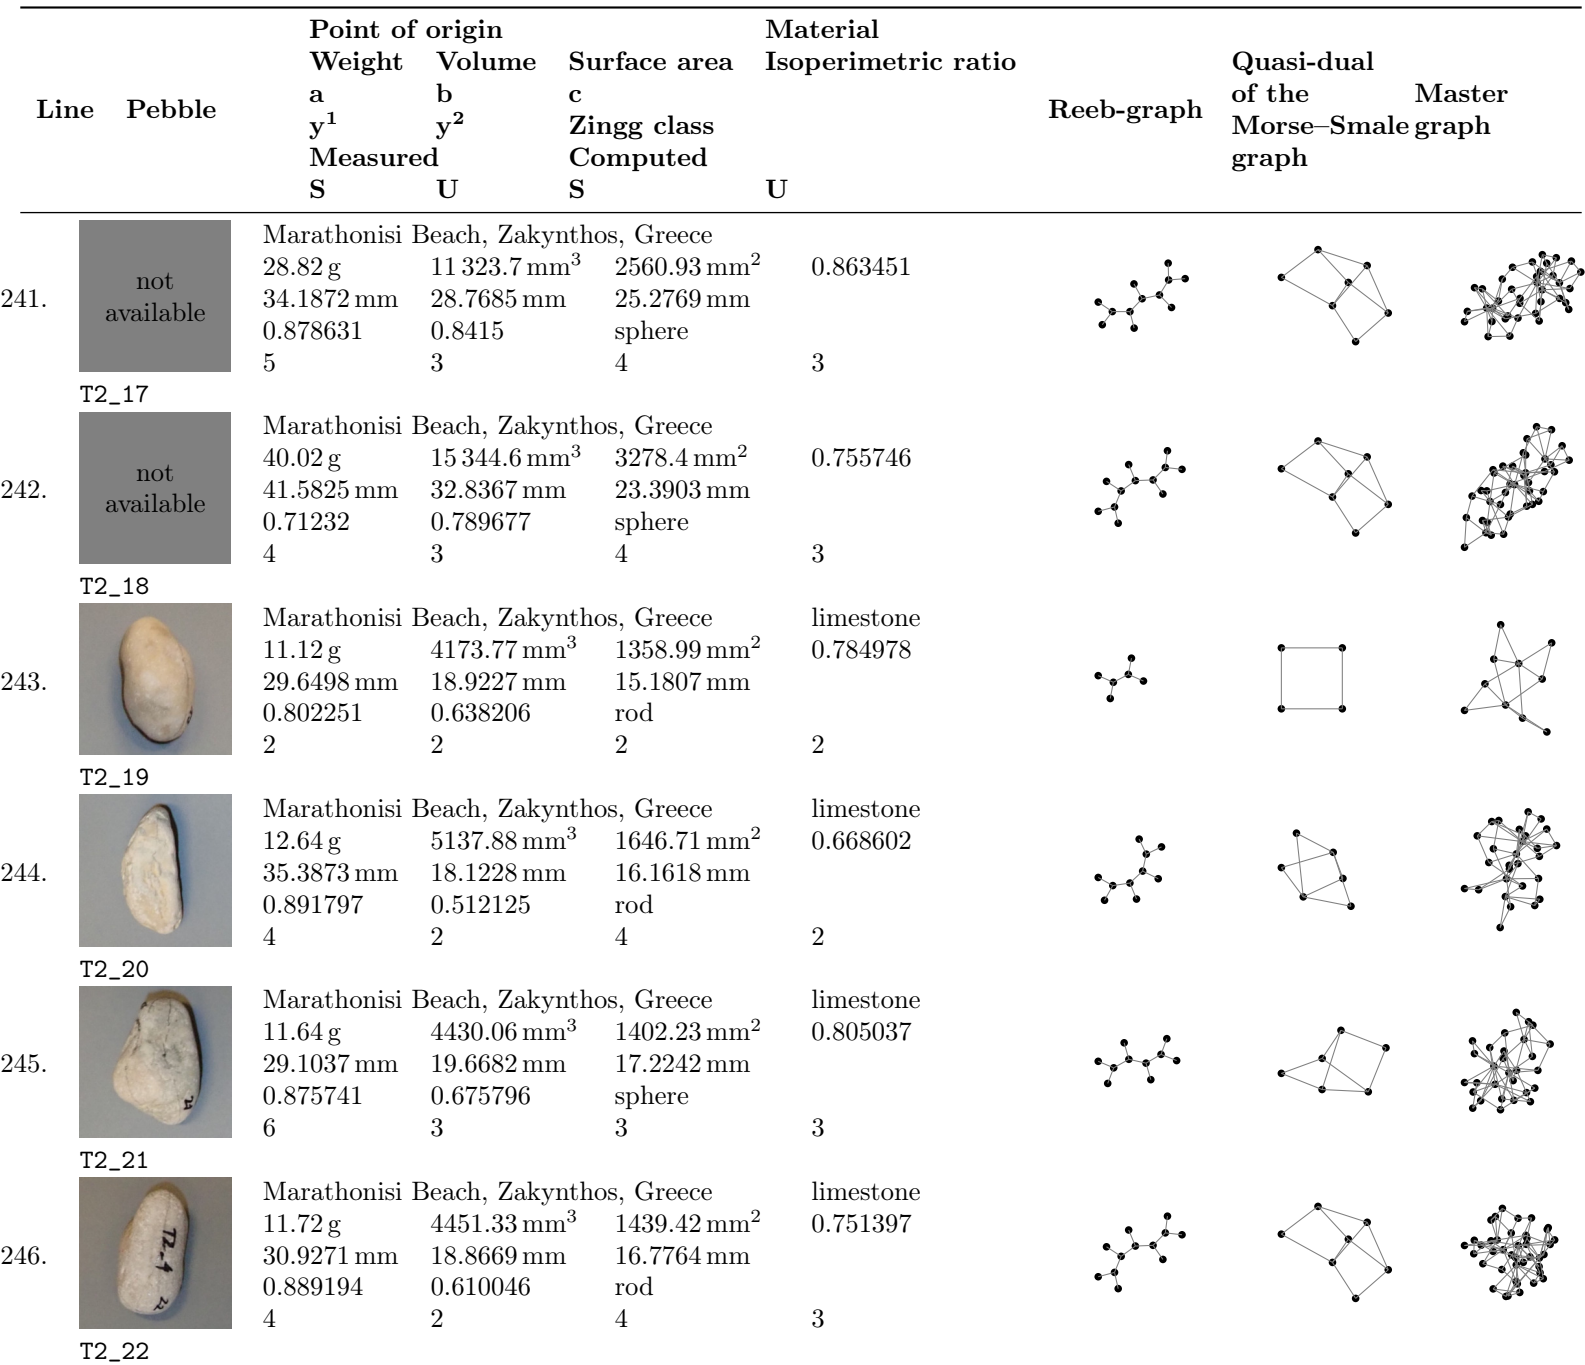 |
|      | T2_21                                                                               |                                                                                |                                                         |                                                      |                                      |                                                                                       |                                                                                       |                                                                                       |
| 246. | 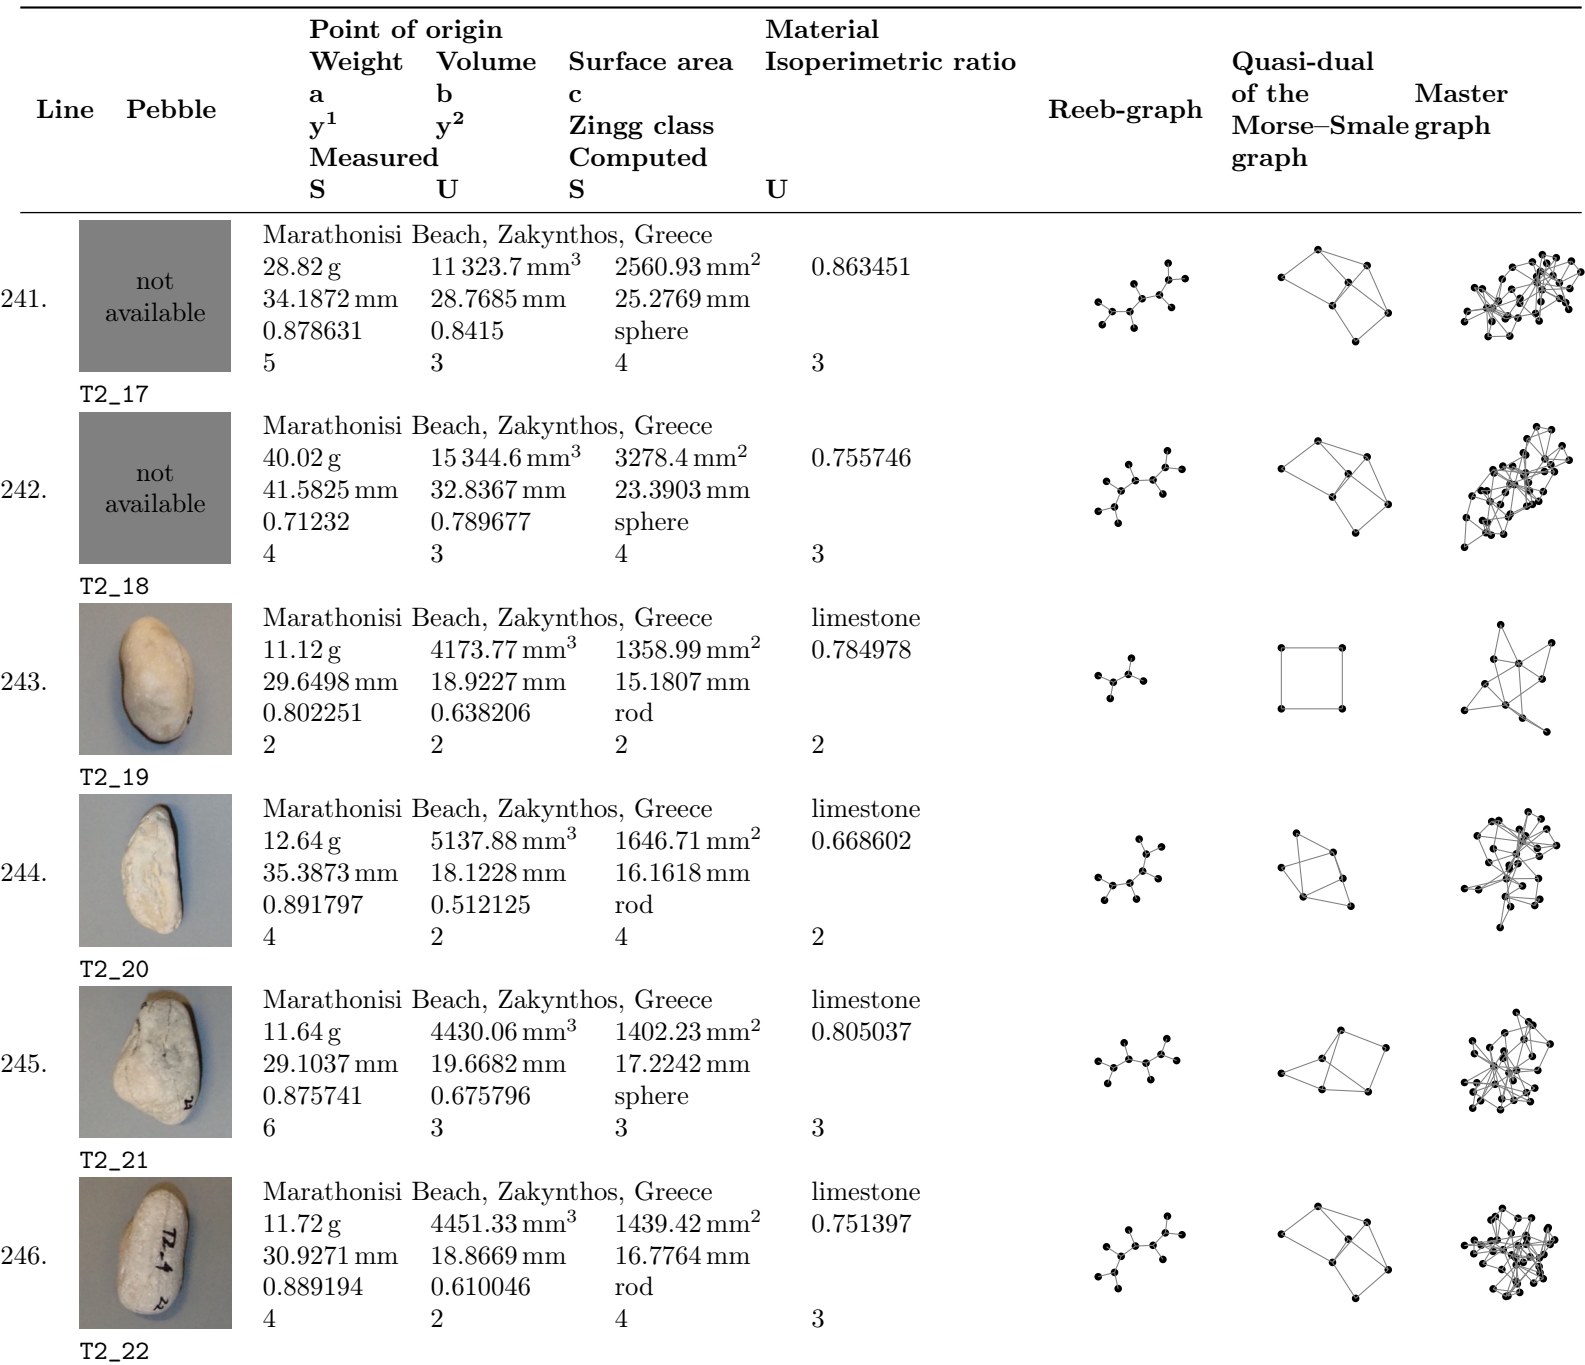 | Marathonisi Beach, Zakynthos, Greece<br>11.72 g<br>30.9271 mm<br>0.889194<br>4 | 4451.33 mm <sup>3</sup><br>18.8669 mm<br>0.610046<br>2  | 1439.42 mm <sup>2</sup><br>16.7764 mm<br>rod<br>4    | limestone<br>0.751397<br><br>3       | 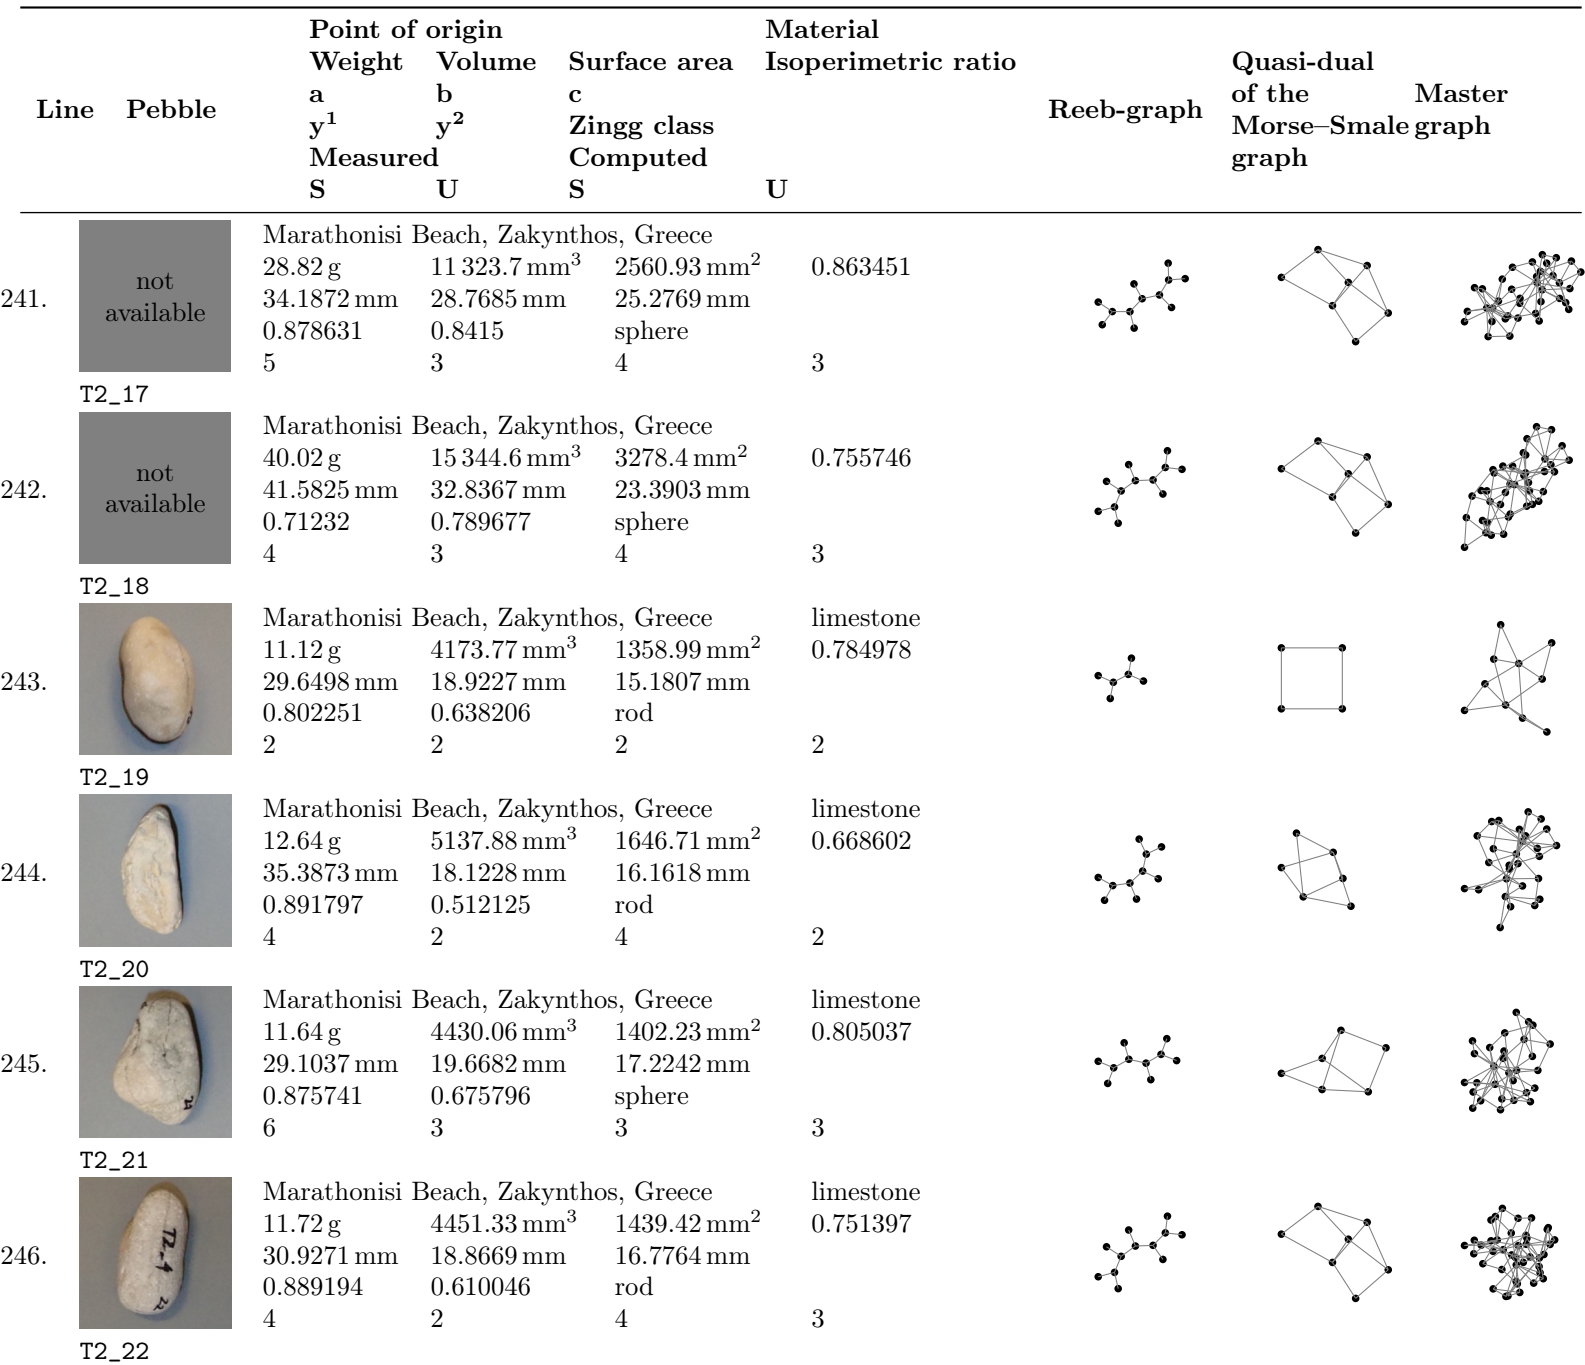 | 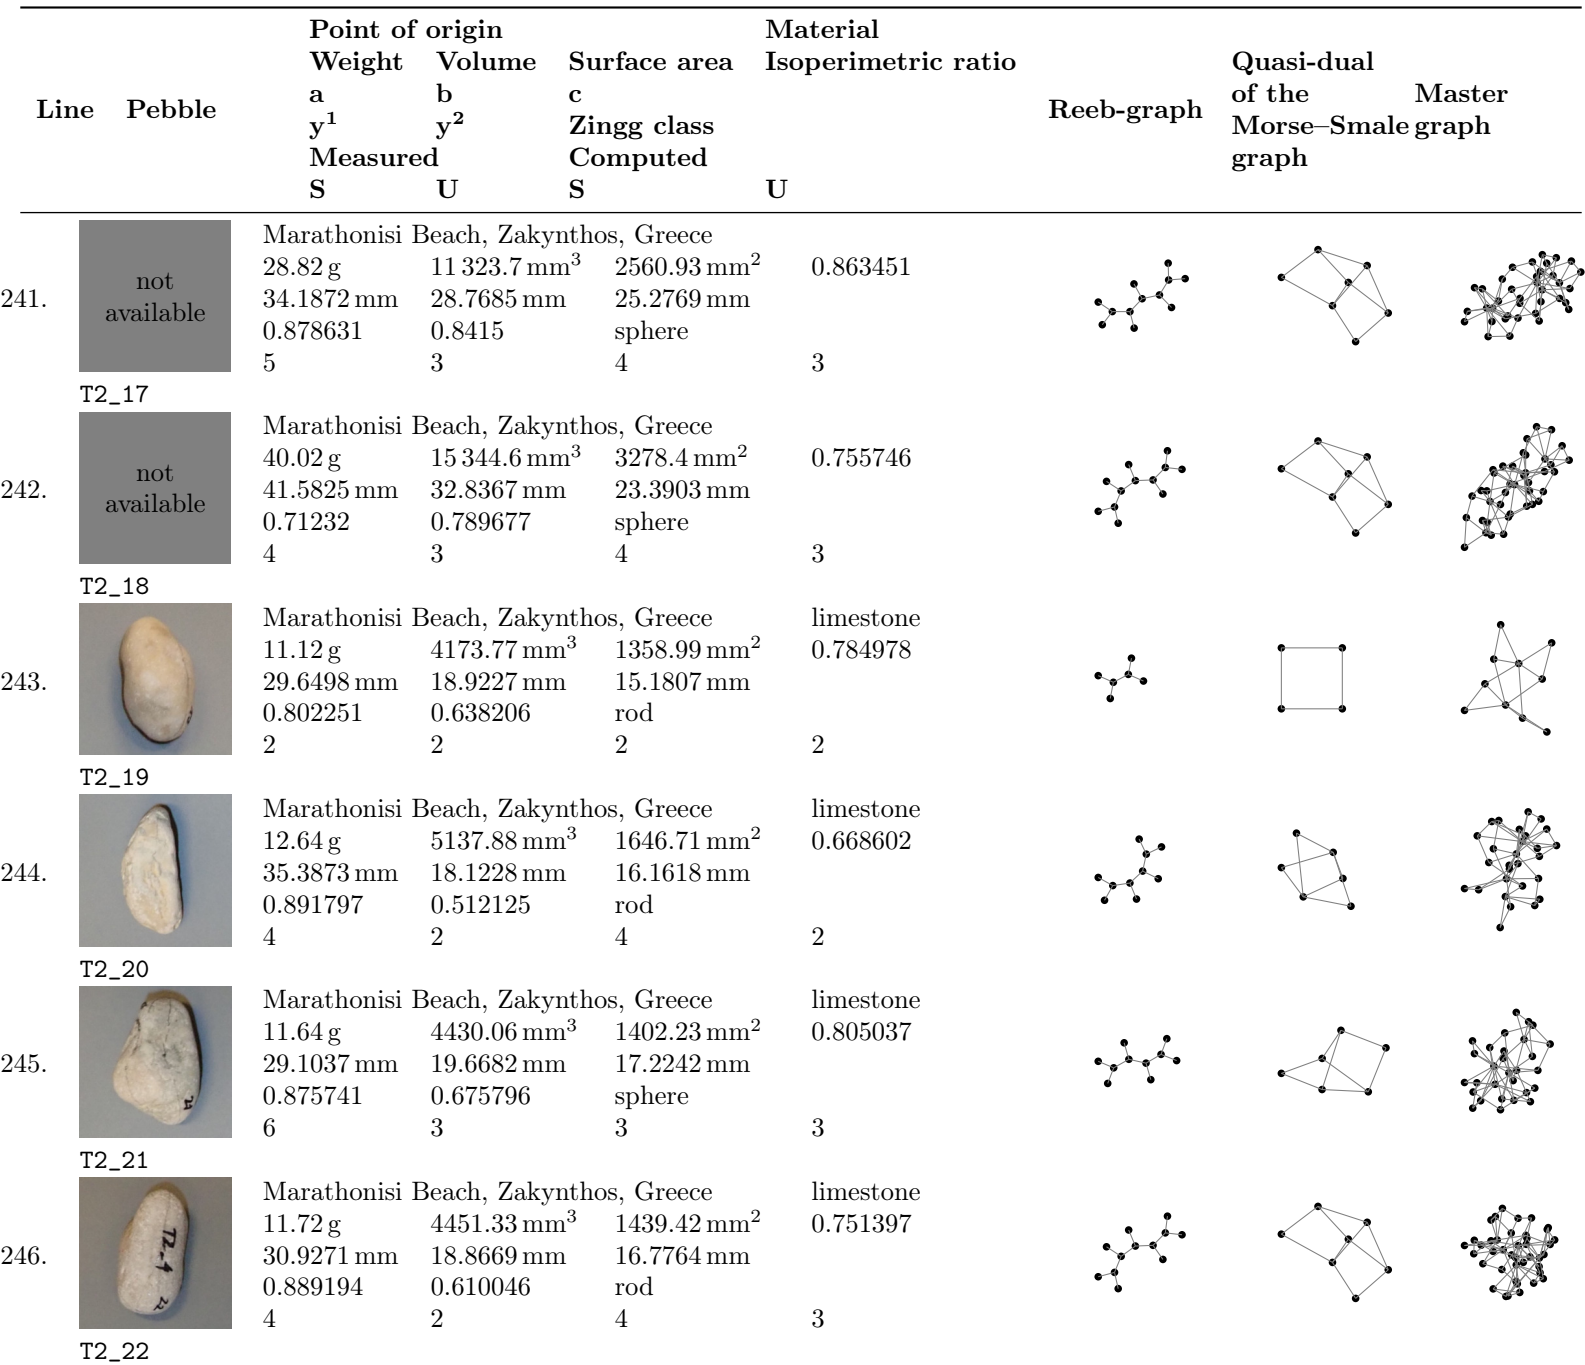 | 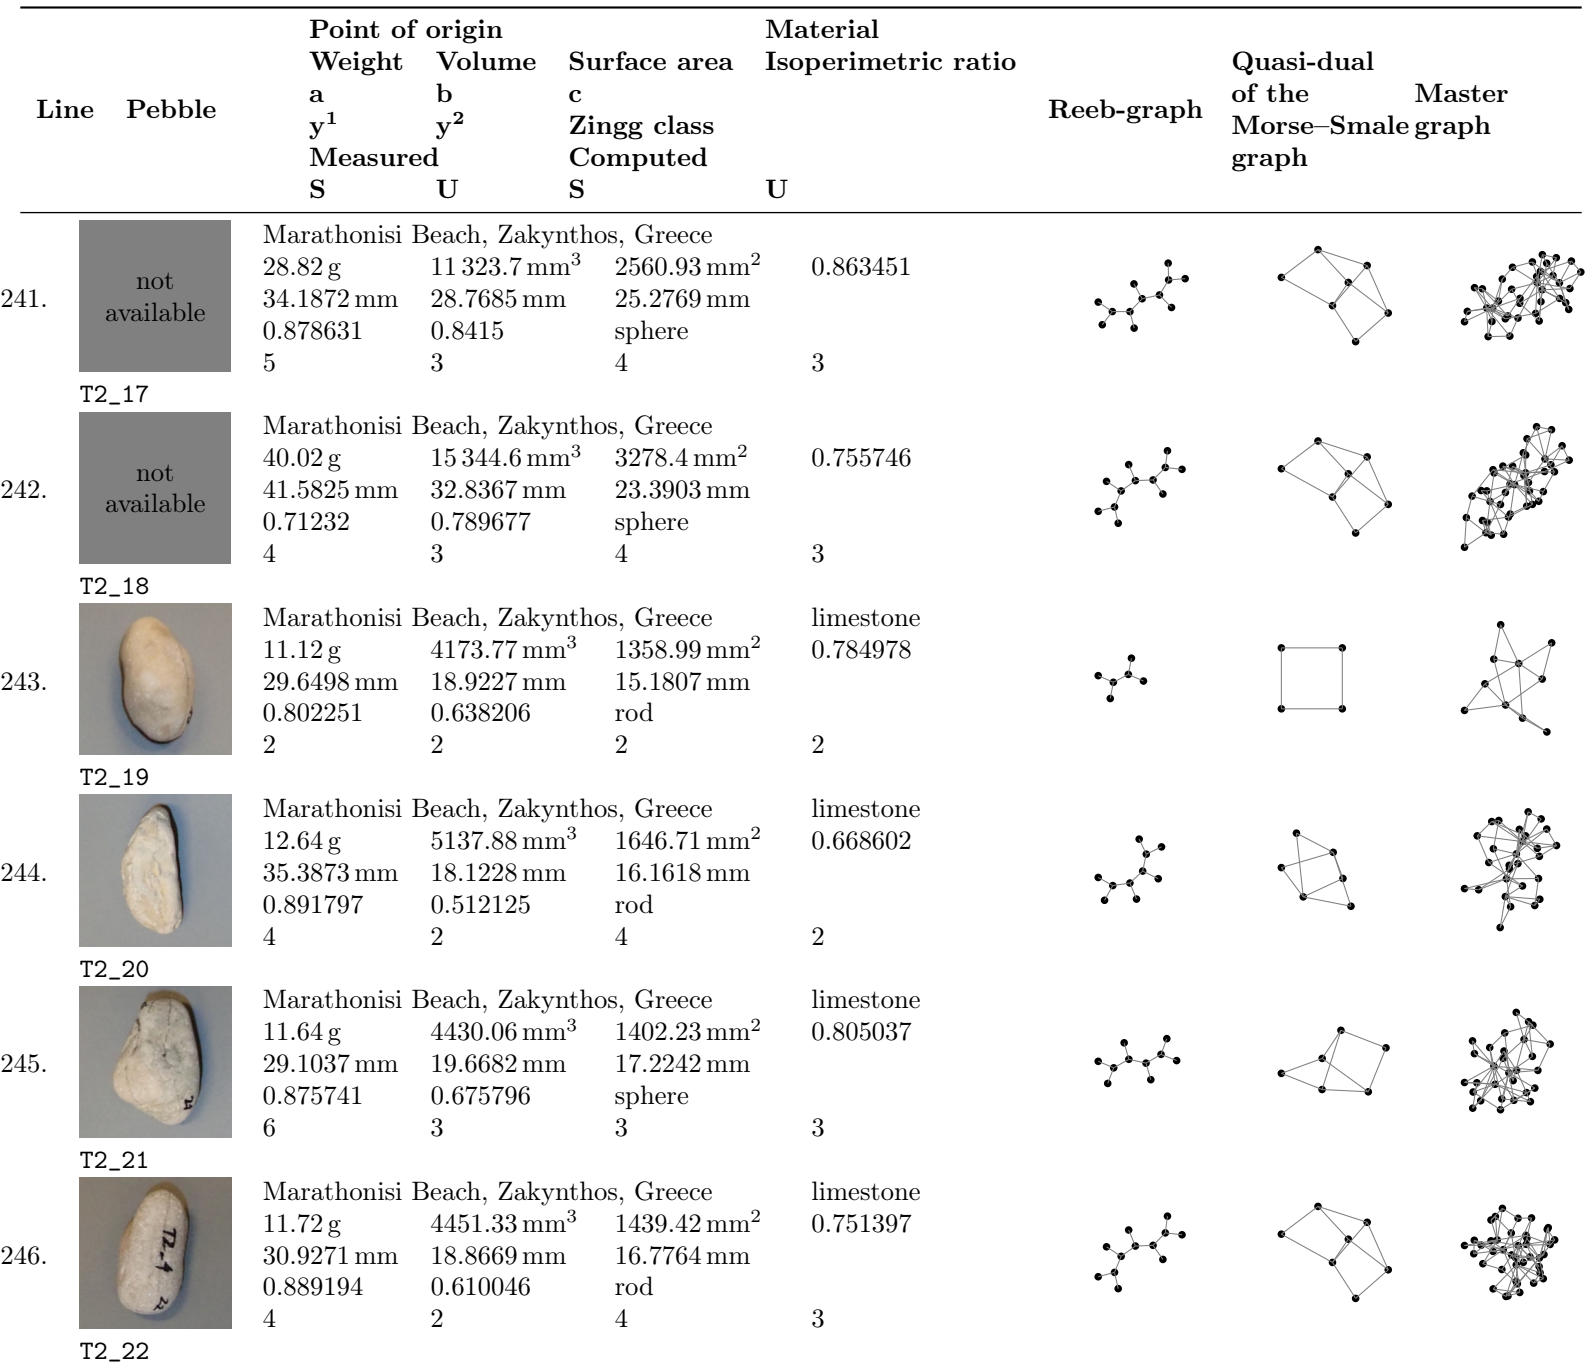 |
|      | T2_22                                                                               |                                                                                |                                                         |                                                      |                                      |                                                                                       |                                                                                       |                                                                                       |

| Line | Pebble                                                                              | Point of origin                      |                          |                              | Material            |   | Reeb-graph | Quasi-dual<br>of the<br>Morse–Smale<br>graph | Master |
|------|-------------------------------------------------------------------------------------|--------------------------------------|--------------------------|------------------------------|---------------------|---|------------|----------------------------------------------|--------|
|      |                                                                                     | Weight                               | Volume                   | Surface area                 | Isoperimetric ratio |   |            |                                              |        |
|      |                                                                                     | a                                    | b                        | c                            |                     |   |            |                                              |        |
|      |                                                                                     | y <sup>1</sup><br>Measured<br>S      | y <sup>2</sup><br>U      | Zingg class<br>Computed<br>S |                     | U |            |                                              |        |
| 247. | 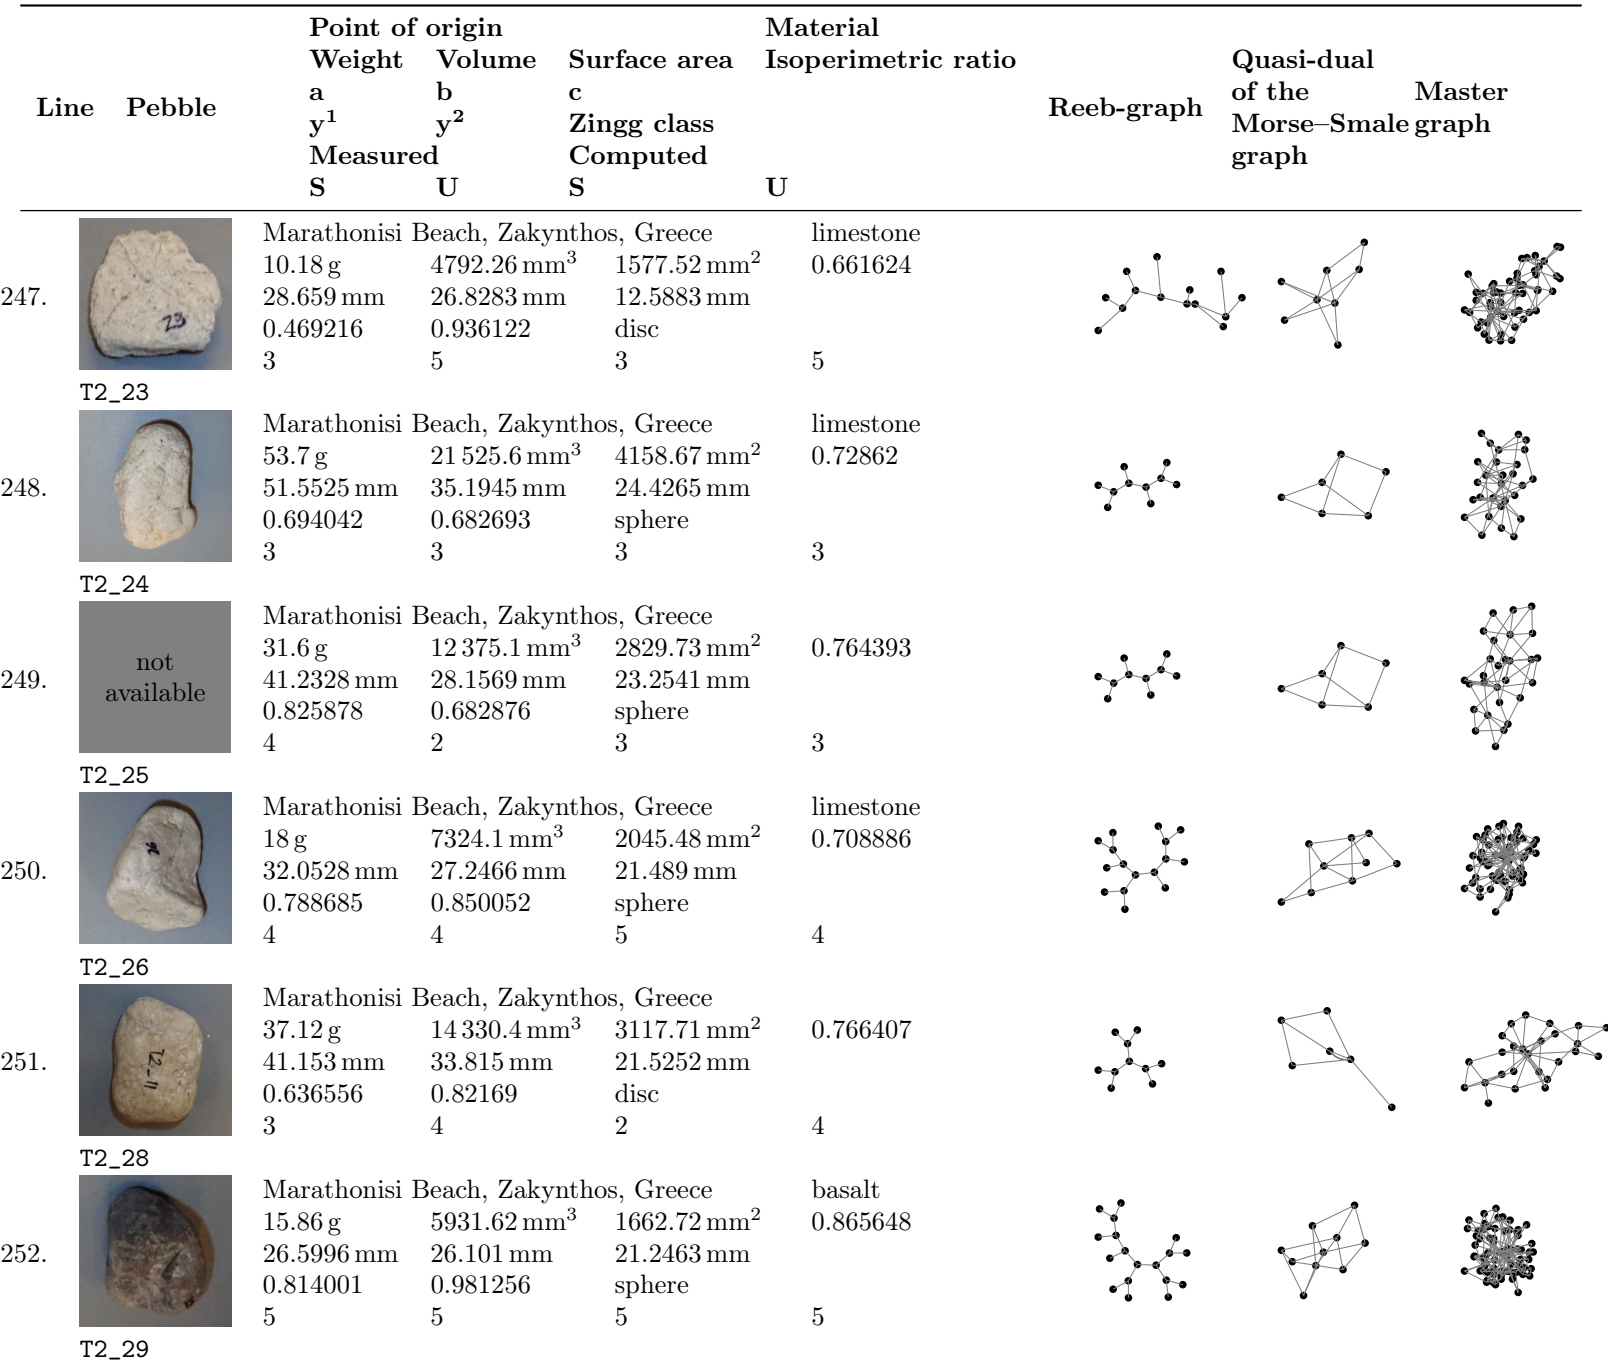   | Marathonisi Beach, Zakynthos, Greece |                          |                              | limestone           |   |            |                                              |        |
|      |                                                                                     | 10.18 g                              | 4792.26 mm <sup>3</sup>  | 1577.52 mm <sup>2</sup>      | 0.661624            |   |            |                                              |        |
|      |                                                                                     | 28.659 mm                            | 26.8283 mm               | 12.5883 mm                   |                     |   |            |                                              |        |
|      |                                                                                     | 0.469216                             | 0.936122                 | disc                         |                     |   |            |                                              |        |
|      |                                                                                     | 3                                    | 5                        | 3                            |                     | 5 |            |                                              |        |
|      | T2_23                                                                               |                                      |                          |                              |                     |   |            |                                              |        |
| 248. | 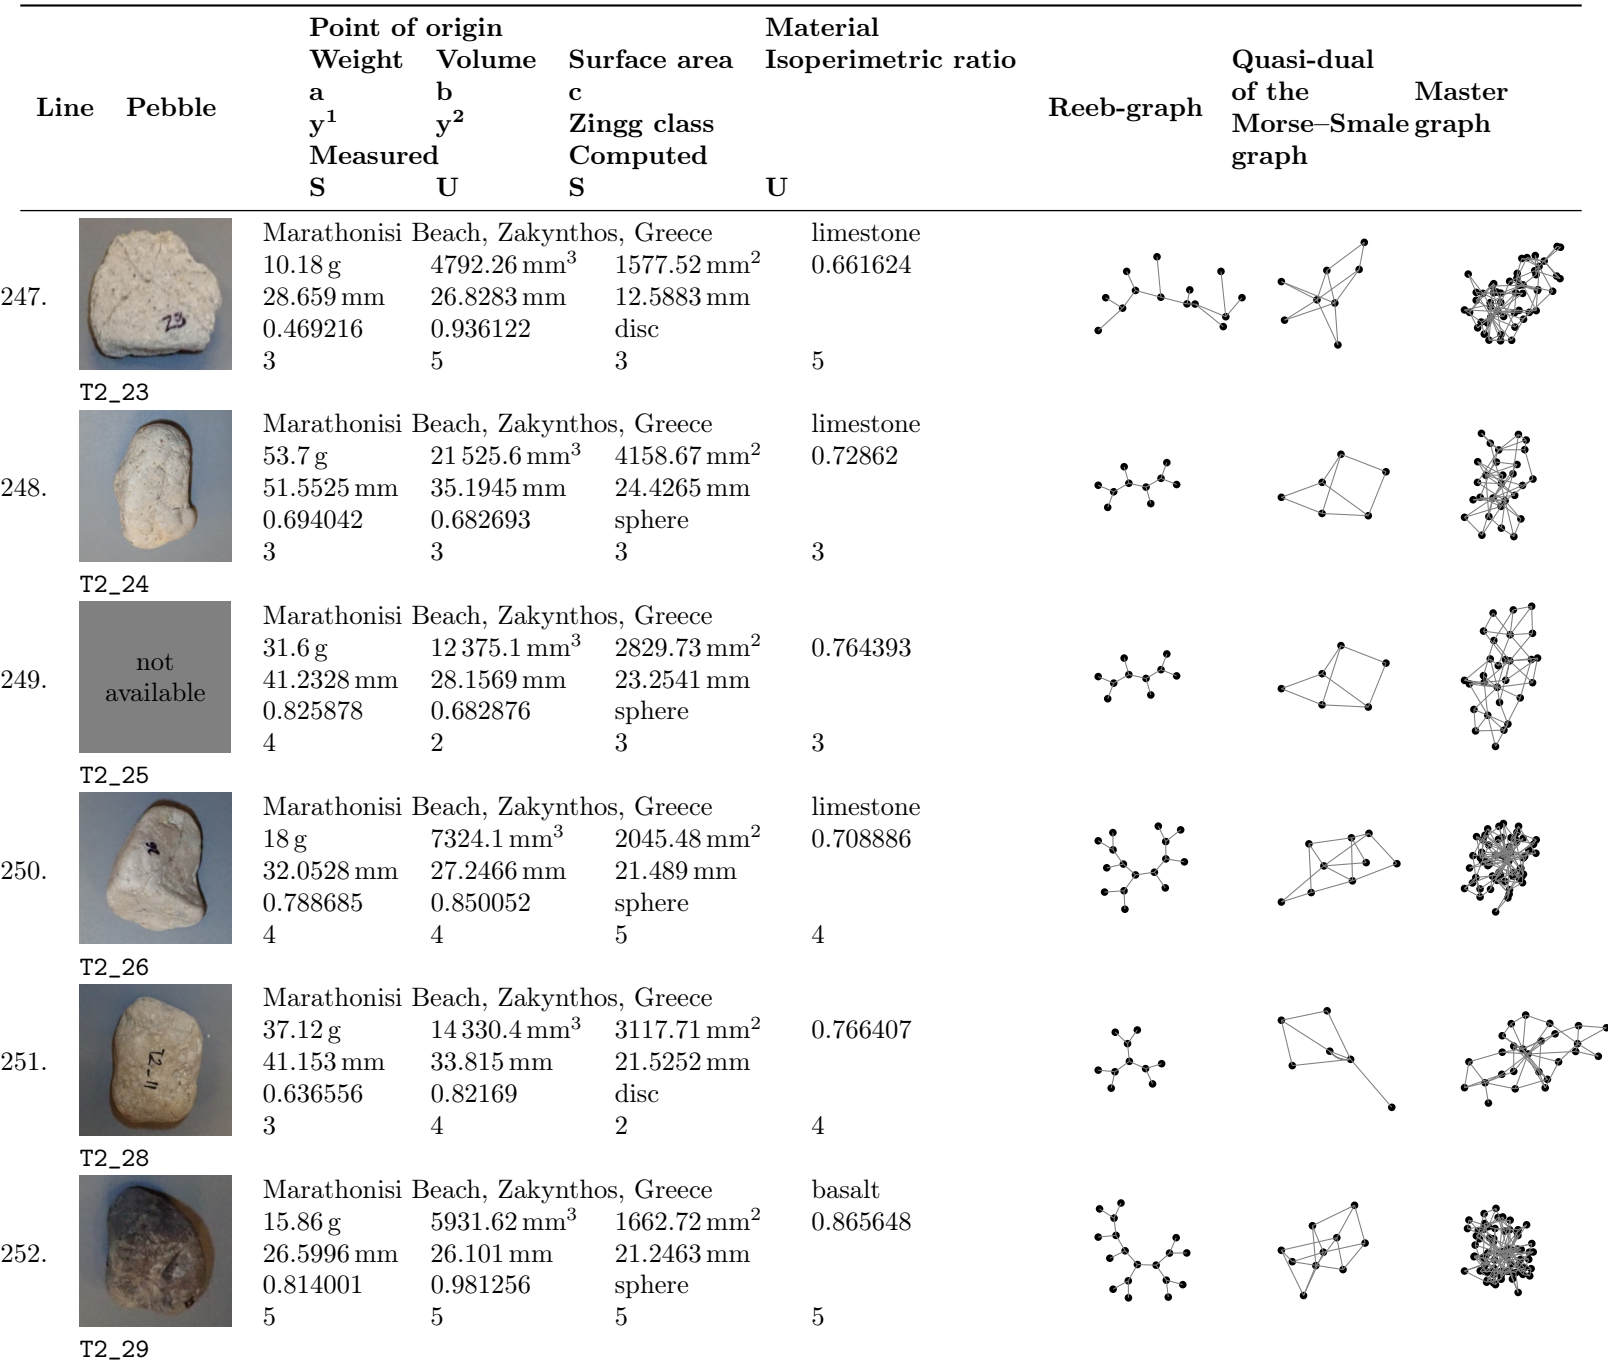   | Marathonisi Beach, Zakynthos, Greece |                          |                              | limestone           |   |            |                                              |        |
|      |                                                                                     | 53.7 g                               | 21 525.6 mm <sup>3</sup> | 4158.67 mm <sup>2</sup>      | 0.72862             |   |            |                                              |        |
|      |                                                                                     | 51.5525 mm                           | 35.1945 mm               | 24.4265 mm                   |                     |   |            |                                              |        |
|      |                                                                                     | 0.694042                             | 0.682693                 | sphere                       |                     |   |            |                                              |        |
|      |                                                                                     | 3                                    | 3                        | 3                            |                     | 3 |            |                                              |        |
|      | T2_24                                                                               |                                      |                          |                              |                     |   |            |                                              |        |
| 249. | 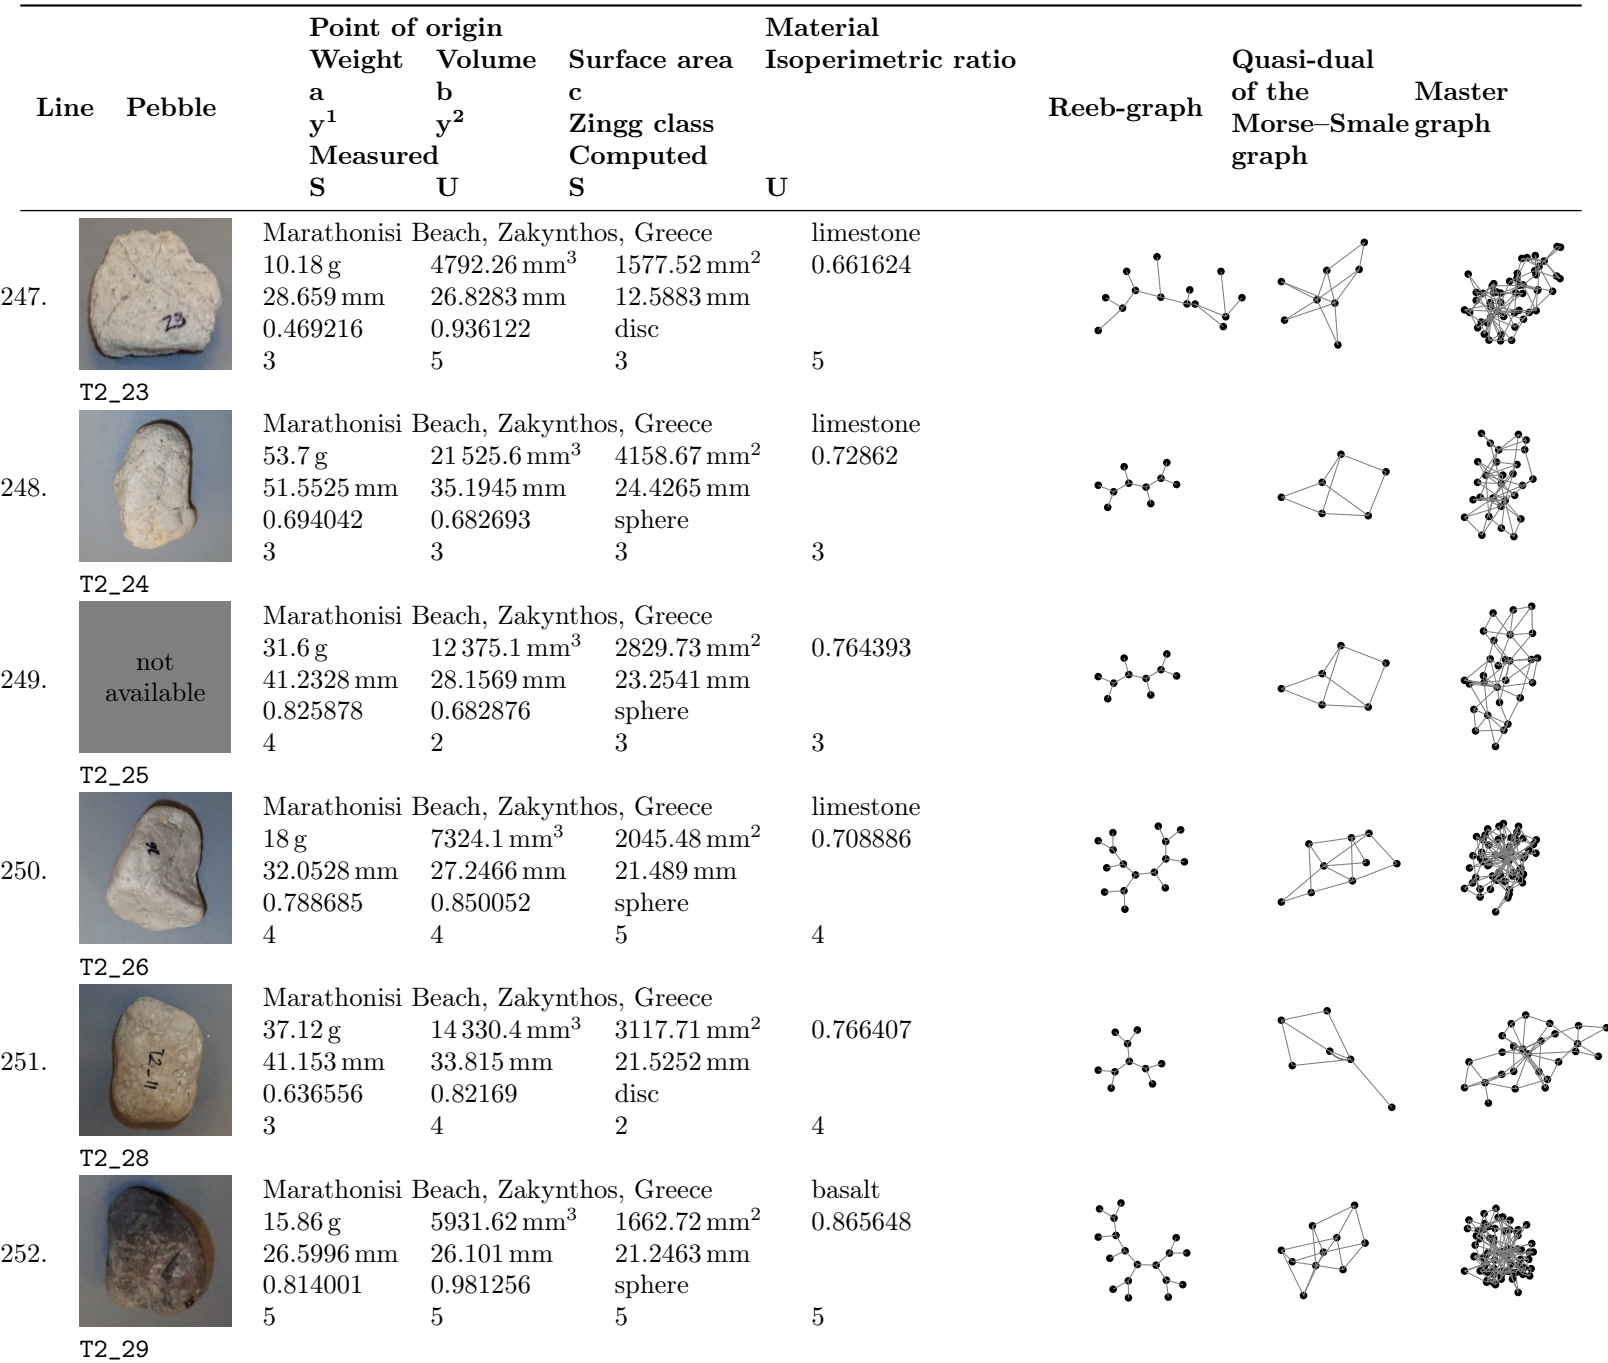   | Marathonisi Beach, Zakynthos, Greece |                          |                              |                     |   |            |                                              |        |
|      |                                                                                     | 31.6 g                               | 12 375.1 mm <sup>3</sup> | 2829.73 mm <sup>2</sup>      | 0.764393            |   |            |                                              |        |
|      |                                                                                     | 41.2328 mm                           | 28.1569 mm               | 23.2541 mm                   |                     |   |            |                                              |        |
|      |                                                                                     | 0.825878                             | 0.682876                 | sphere                       |                     |   |            |                                              |        |
|      |                                                                                     | 4                                    | 2                        | 3                            |                     | 3 |            |                                              |        |
|      | T2_25                                                                               |                                      |                          |                              |                     |   |            |                                              |        |
| 250. | 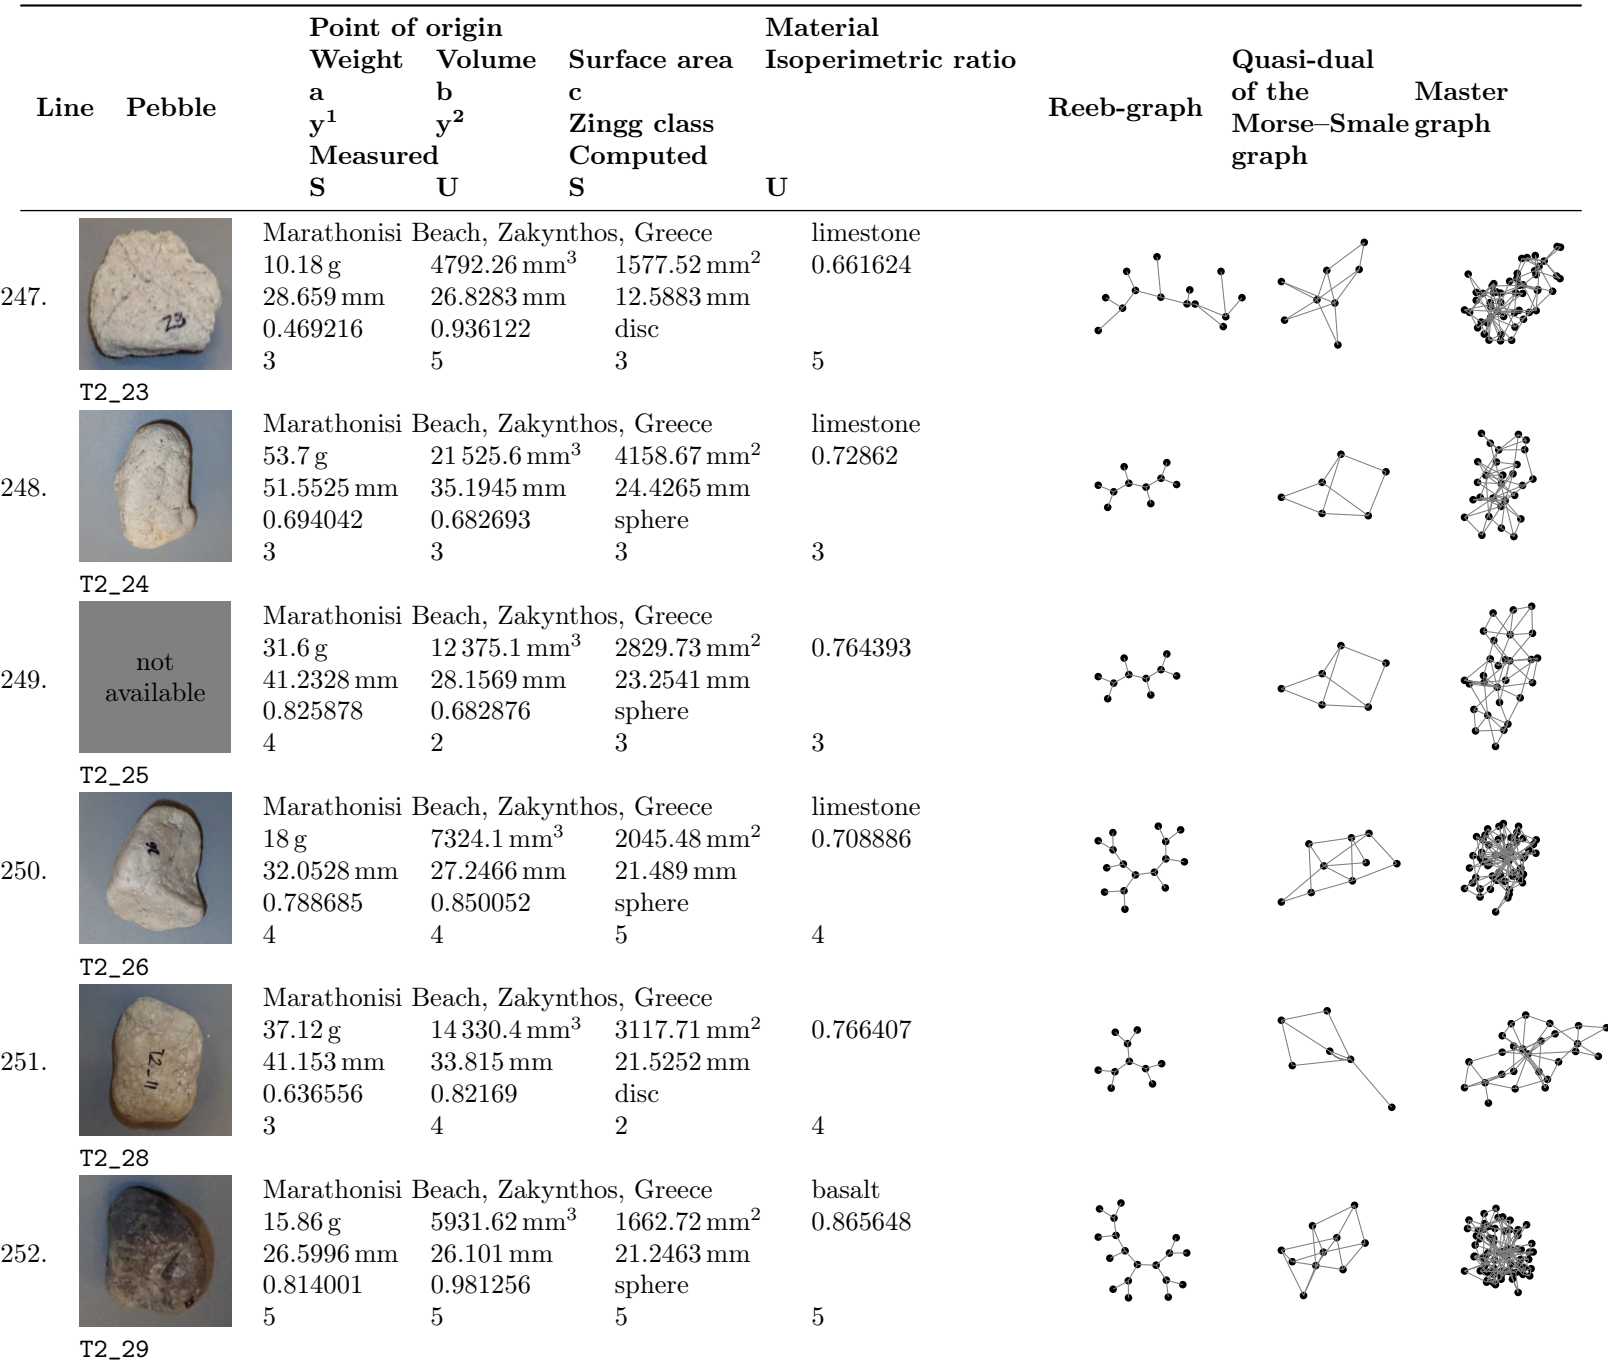  | Marathonisi Beach, Zakynthos, Greece |                          |                              | limestone           |   |            |                                              |        |
|      |                                                                                     | 18 g                                 | 7324.1 mm <sup>3</sup>   | 2045.48 mm <sup>2</sup>      | 0.708886            |   |            |                                              |        |
|      |                                                                                     | 32.0528 mm                           | 27.2466 mm               | 21.489 mm                    |                     |   |            |                                              |        |
|      |                                                                                     | 0.788685                             | 0.850052                 | sphere                       |                     |   |            |                                              |        |
|      |                                                                                     | 4                                    | 4                        | 5                            |                     | 4 |            |                                              |        |
|      | T2_26                                                                               |                                      |                          |                              |                     |   |            |                                              |        |
| 251. | 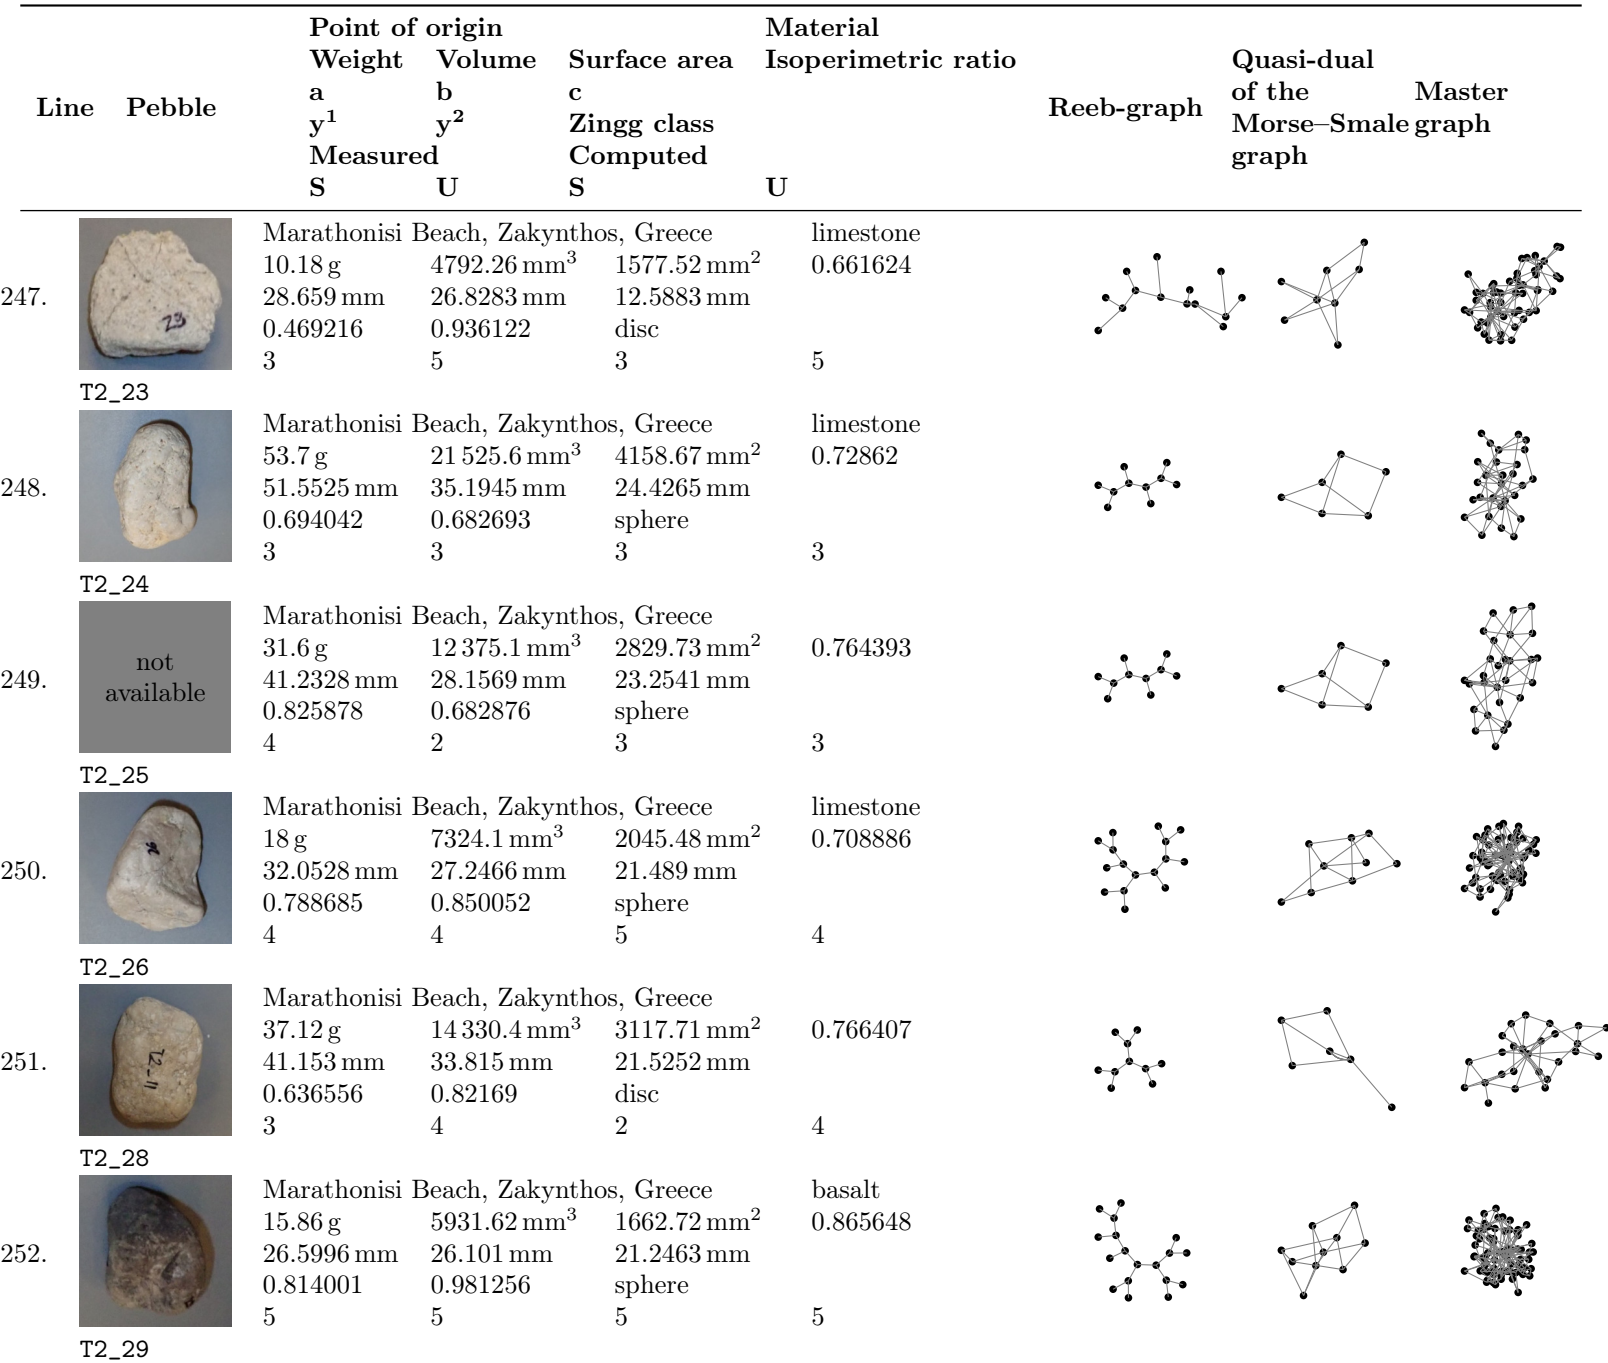 | Marathonisi Beach, Zakynthos, Greece |                          |                              |                     |   |            |                                              |        |
|      |                                                                                     | 37.12 g                              | 14 330.4 mm <sup>3</sup> | 3117.71 mm <sup>2</sup>      | 0.766407            |   |            |                                              |        |
|      |                                                                                     | 41.153 mm                            | 33.815 mm                | 21.5252 mm                   |                     |   |            |                                              |        |
|      |                                                                                     | 0.636556                             | 0.82169                  | disc                         |                     |   |            |                                              |        |
|      |                                                                                     | 3                                    | 4                        | 2                            |                     | 4 |            |                                              |        |
|      | T2_28                                                                               |                                      |                          |                              |                     |   |            |                                              |        |
| 252. | 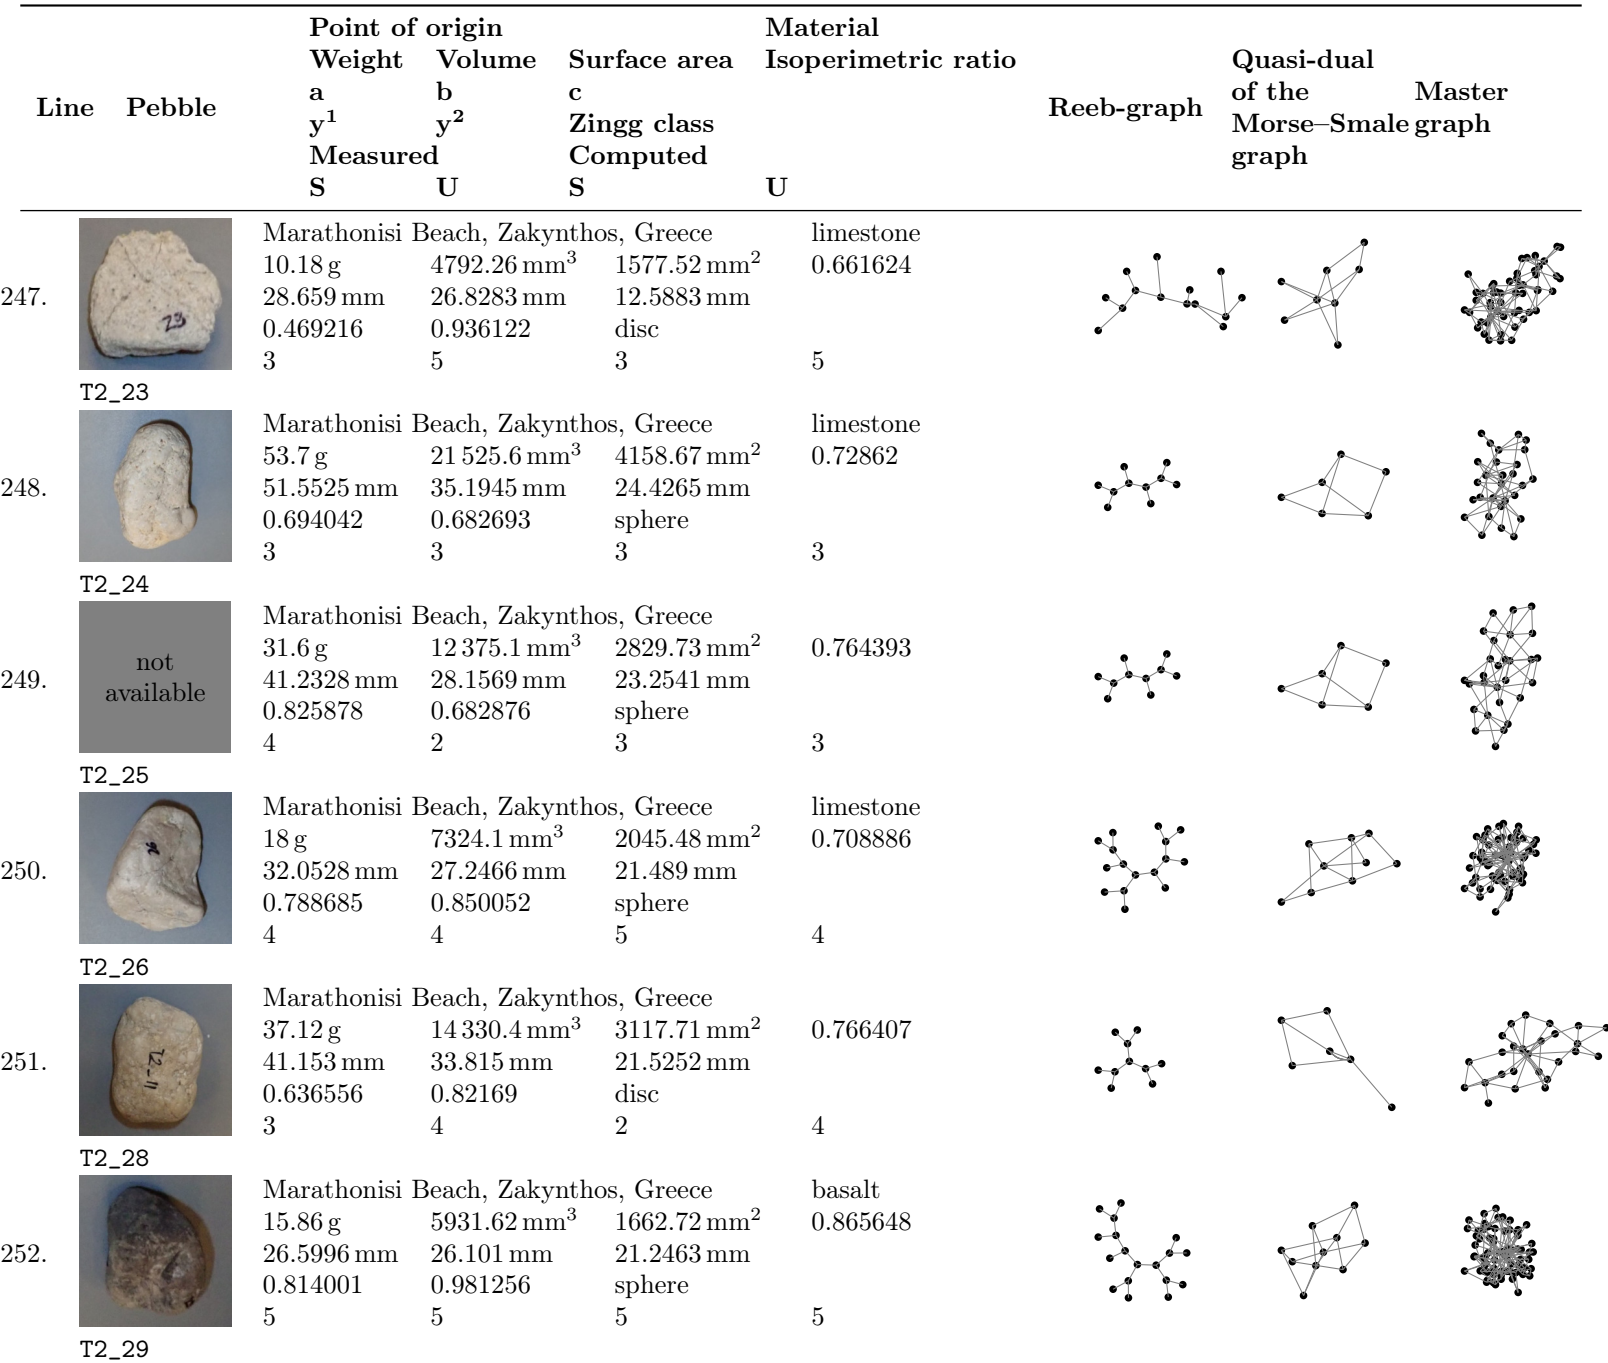 | Marathonisi Beach, Zakynthos, Greece |                          |                              | basalt              |   |            |                                              |        |
|      |                                                                                     | 15.86 g                              | 5931.62 mm <sup>3</sup>  | 1662.72 mm <sup>2</sup>      | 0.865648            |   |            |                                              |        |
|      |                                                                                     | 26.5996 mm                           | 26.101 mm                | 21.2463 mm                   |                     |   |            |                                              |        |
|      |                                                                                     | 0.814001                             | 0.981256                 | sphere                       |                     |   |            |                                              |        |
|      |                                                                                     | 5                                    | 5                        | 5                            |                     | 5 |            |                                              |        |
|      | T2_29                                                                               |                                      |                          |                              |                     |   |            |                                              |        |

| Line | Pebble                                                                              | Point of origin                                                                |                                                                    | Surface area<br>c<br>Zingg class<br>Computed<br>S    | Material<br>Isoperimetric ratio<br>U | Reeb-graph                                                                            | Quasi-dual<br>of the<br>Morse–Smale<br>graph                                          | Master<br>graph                                                                       |
|------|-------------------------------------------------------------------------------------|--------------------------------------------------------------------------------|--------------------------------------------------------------------|------------------------------------------------------|--------------------------------------|---------------------------------------------------------------------------------------|---------------------------------------------------------------------------------------|---------------------------------------------------------------------------------------|
|      |                                                                                     | Weight                                                                         | Volume                                                             |                                                      |                                      |                                                                                       |                                                                                       |                                                                                       |
|      |                                                                                     | a<br>y <sup>1</sup><br>Measured<br>S                                           | b<br>y <sup>2</sup><br>U                                           |                                                      |                                      |                                                                                       |                                                                                       |                                                                                       |
|      |                                                                                     |                                                                                |                                                                    |                                                      |                                      |                                                                                       |                                                                                       |                                                                                       |
| 253. | 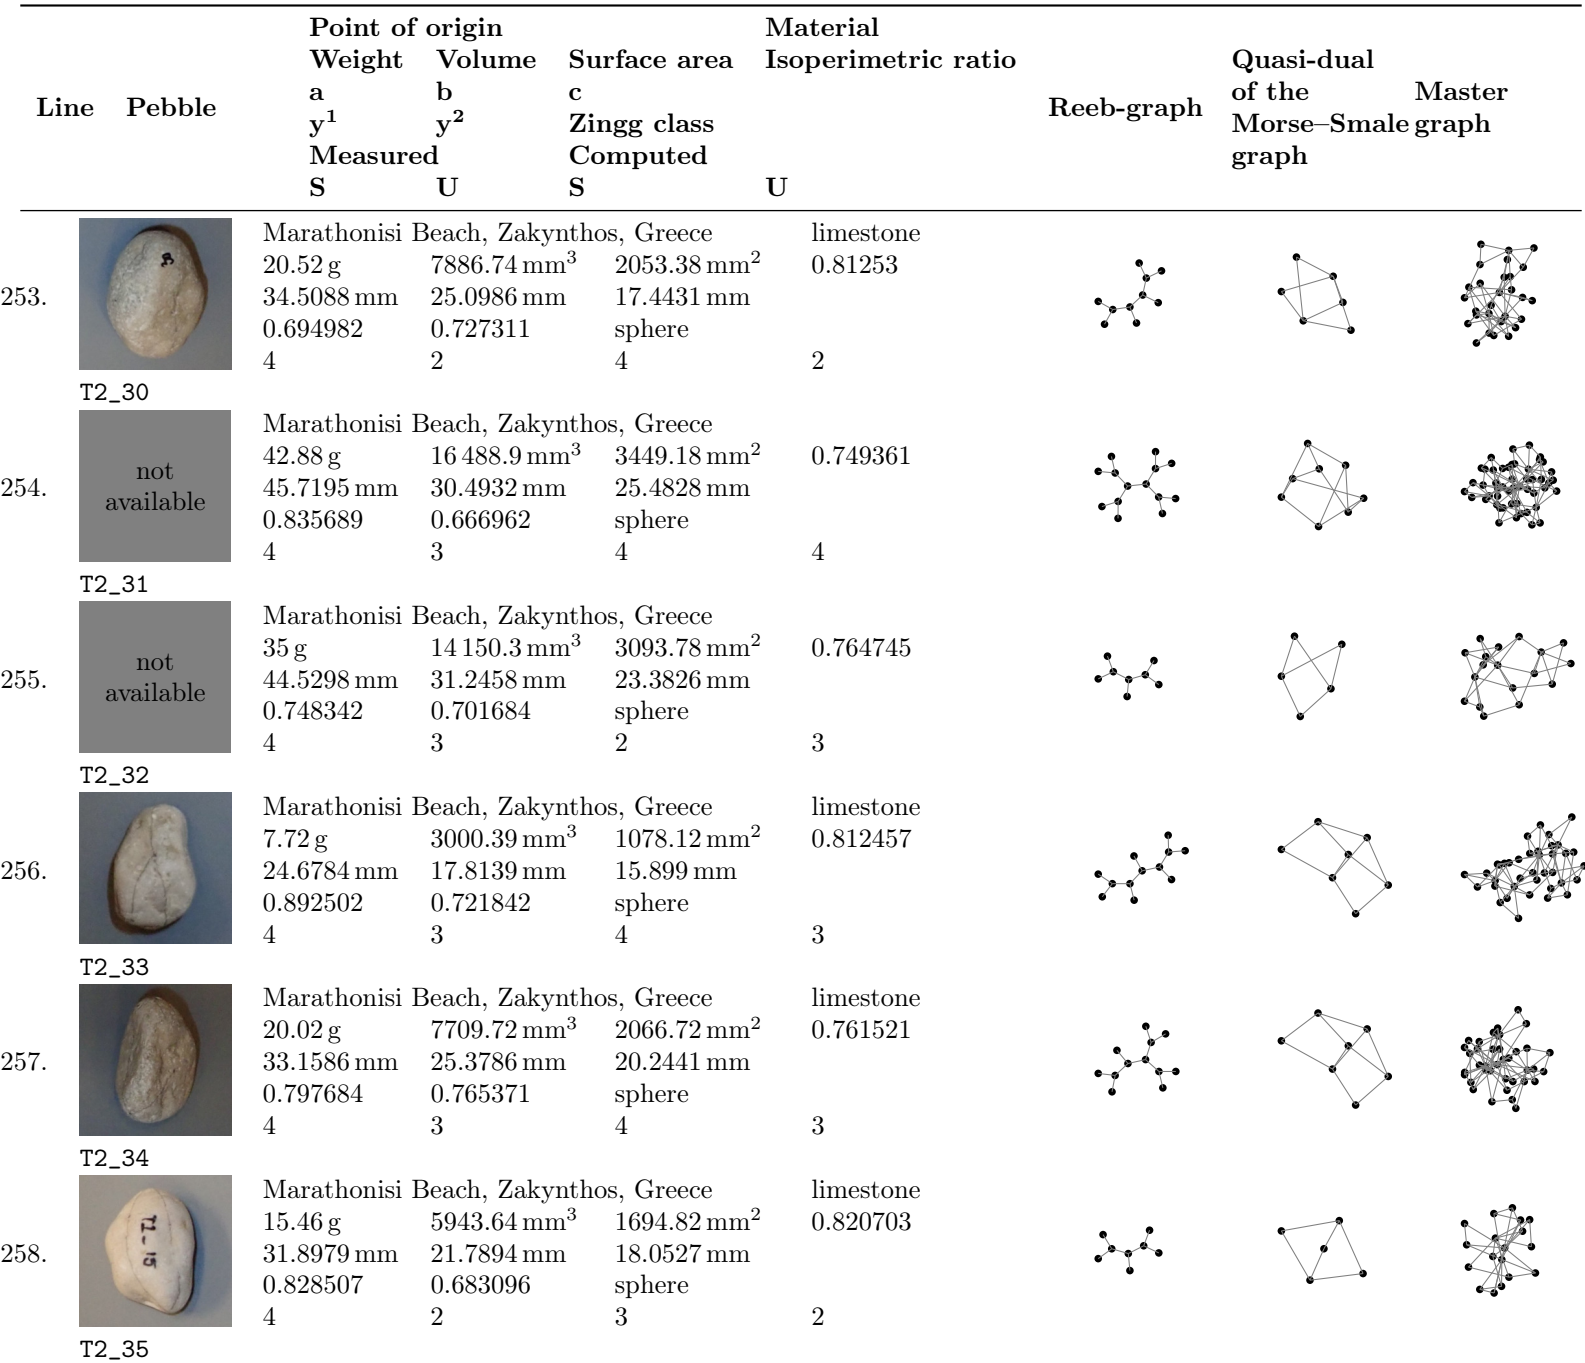   | Marathonisi Beach, Zakynthos, Greece<br>20.52 g<br>34.5088 mm<br>0.694982<br>4 | 20.52 g<br>7886.74 mm <sup>3</sup><br>25.0986 mm<br>0.727311<br>2  | 2053.38 mm <sup>2</sup><br>17.4431 mm<br>sphere<br>4 | limestone<br>0.81253<br><br>2        | 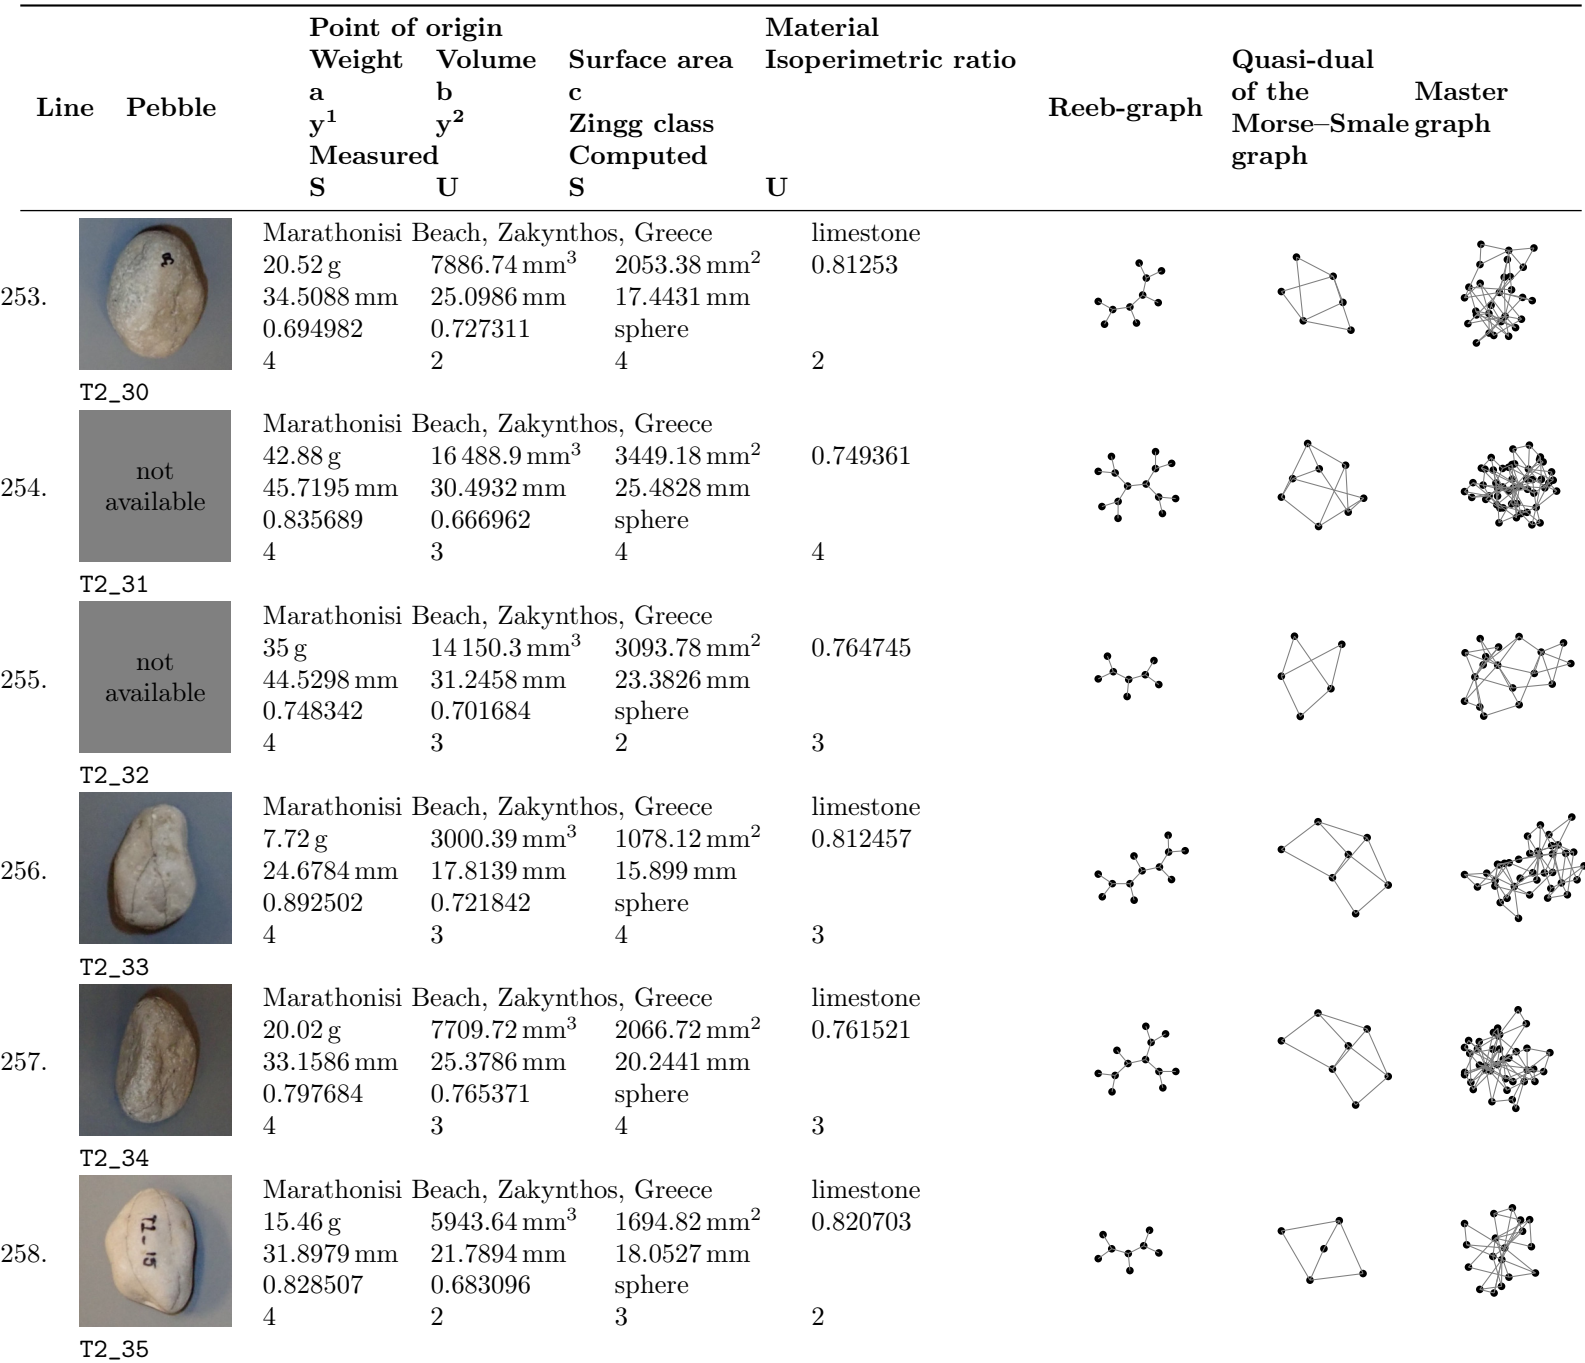   | 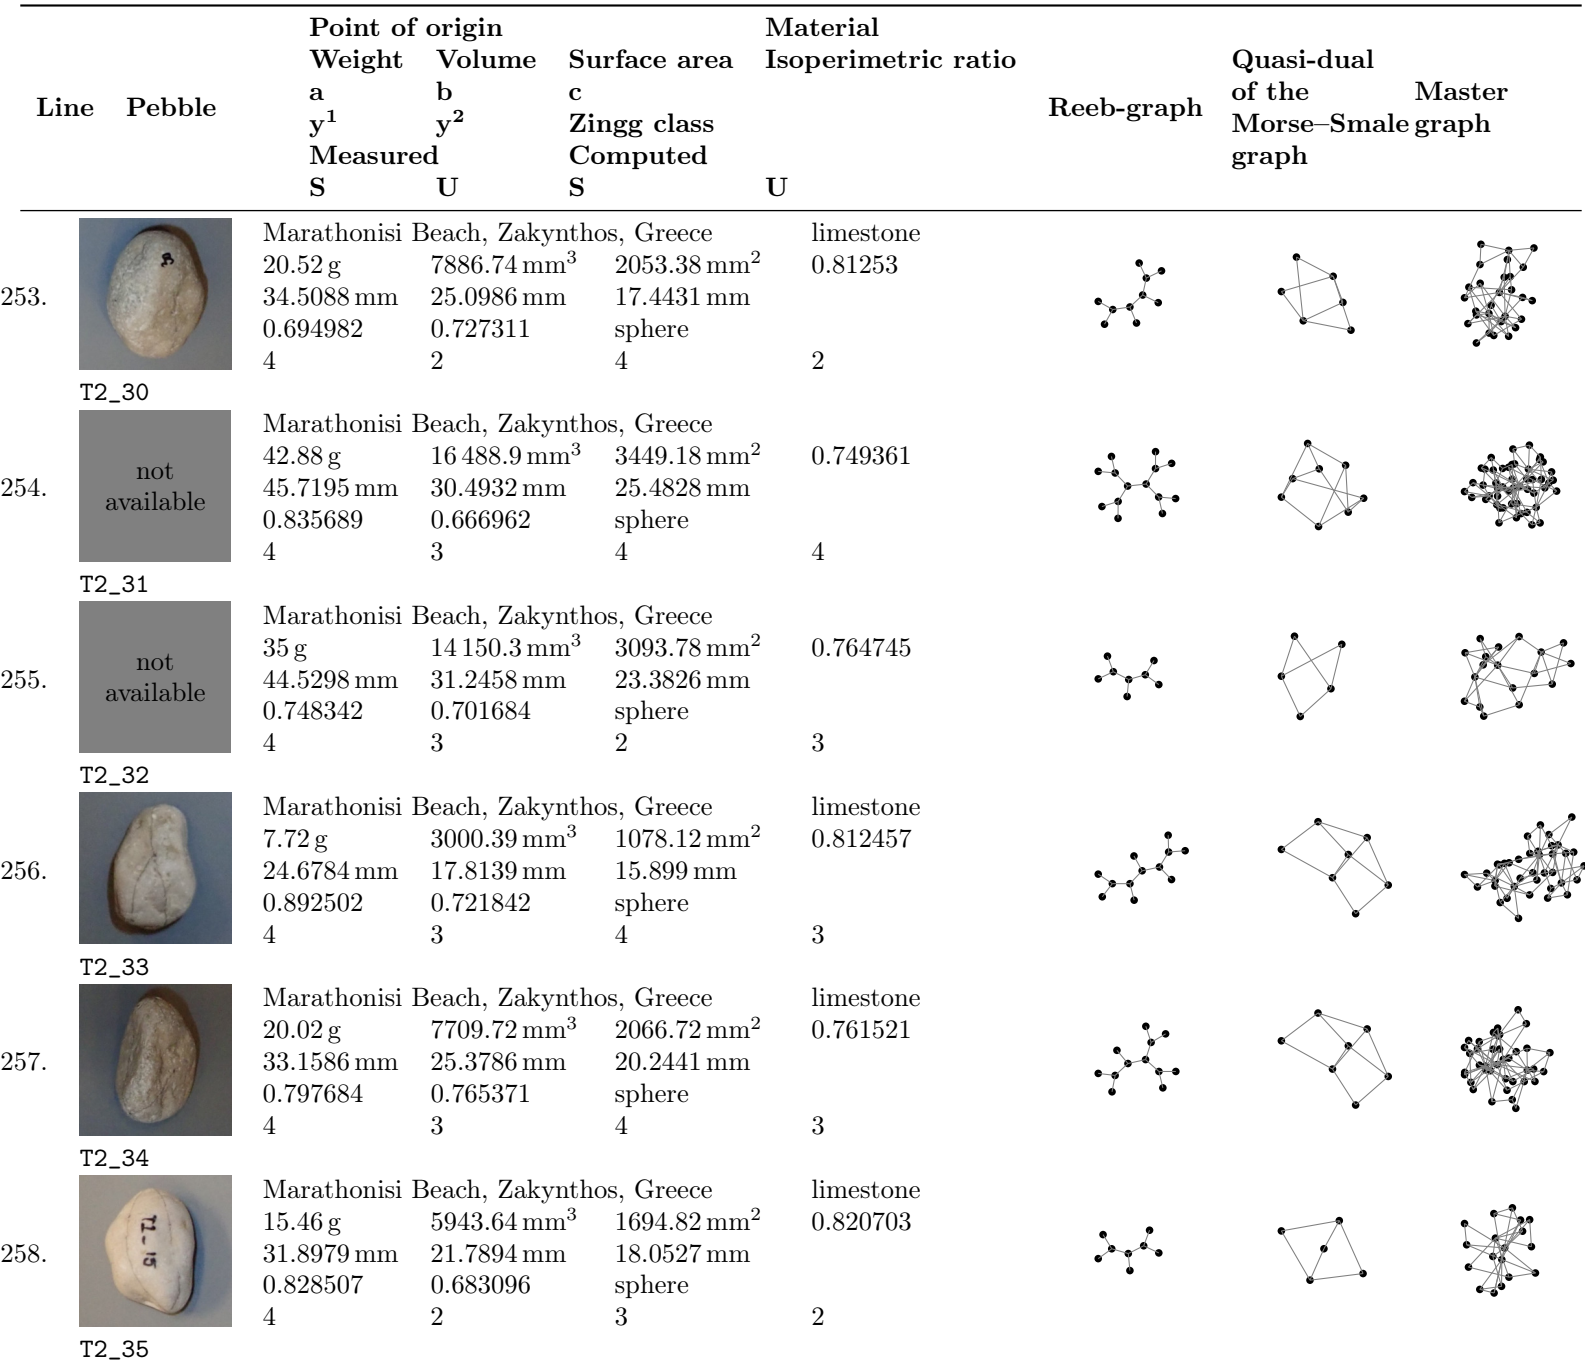   | 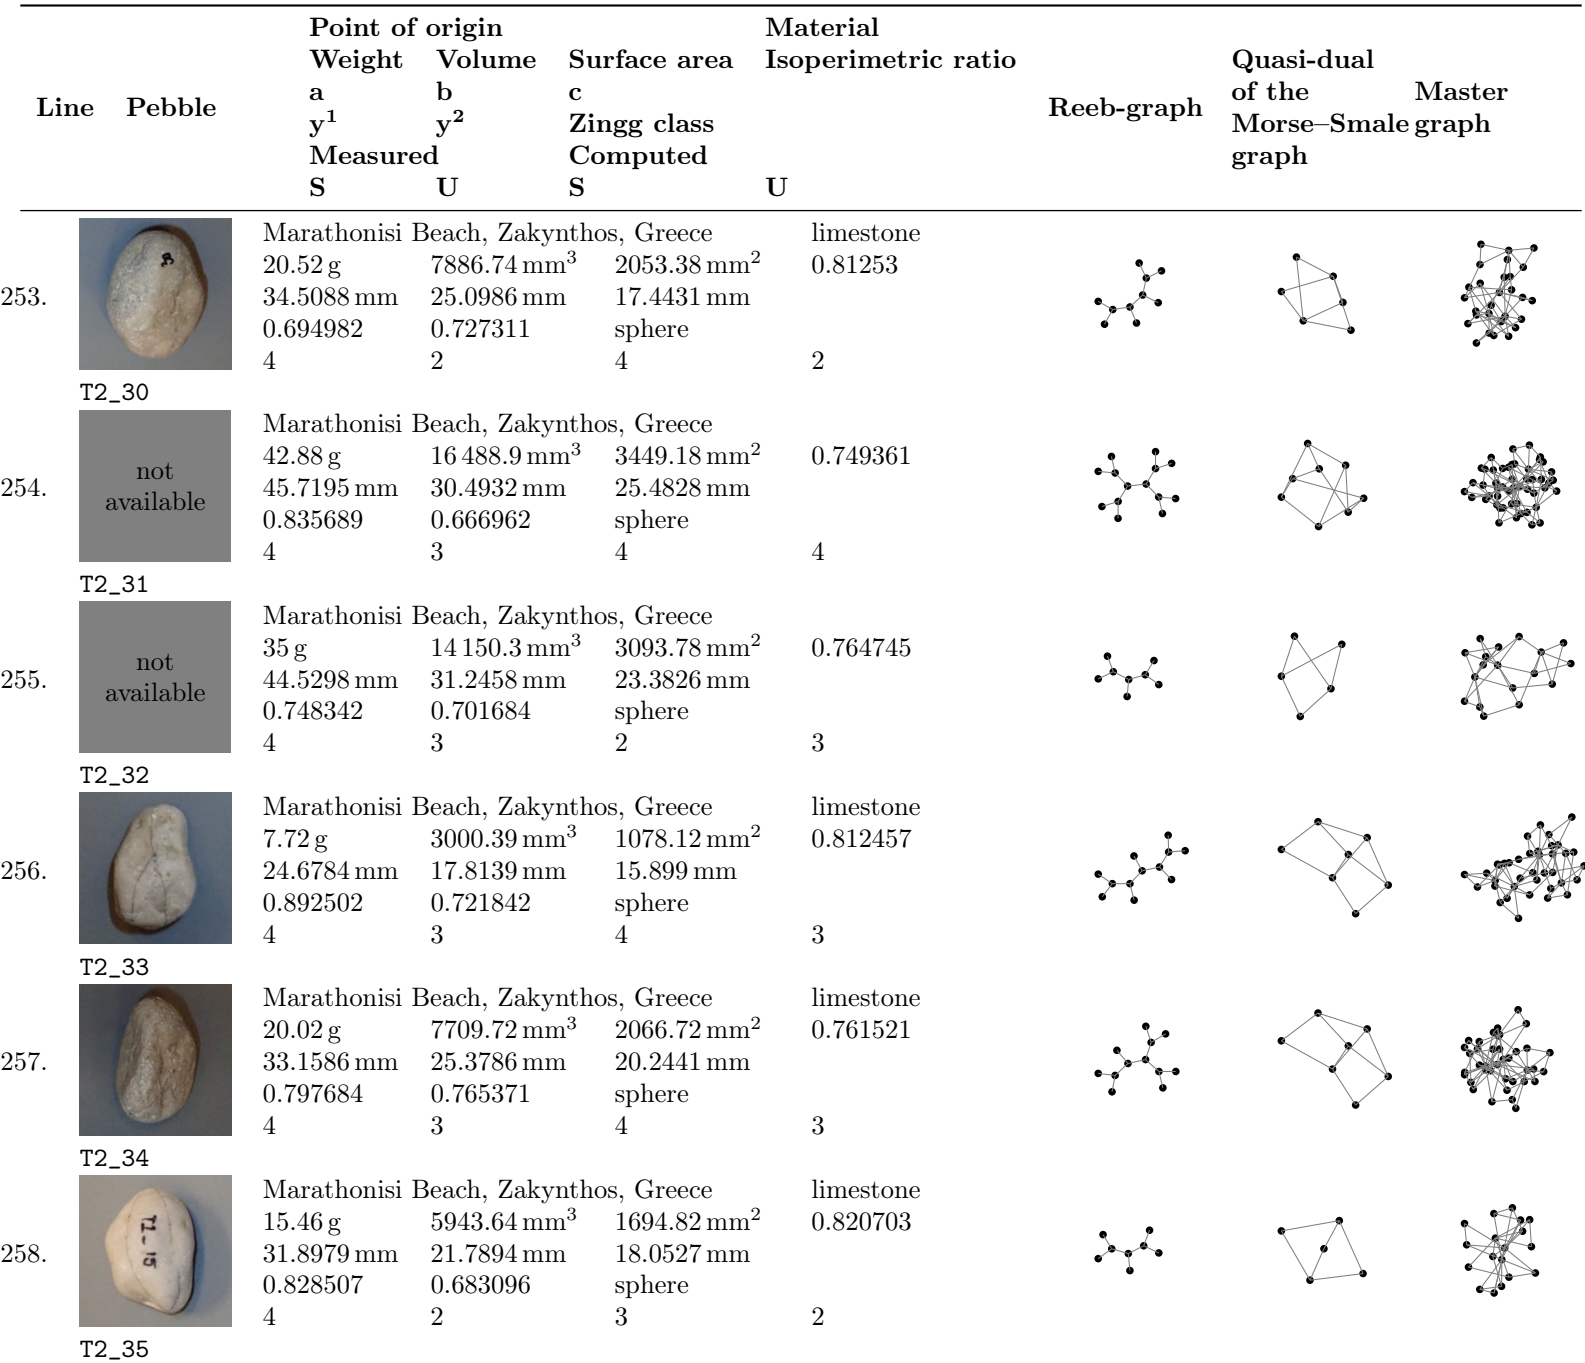   |
|      | T2_30                                                                               |                                                                                |                                                                    |                                                      |                                      |                                                                                       |                                                                                       |                                                                                       |
| 254. | 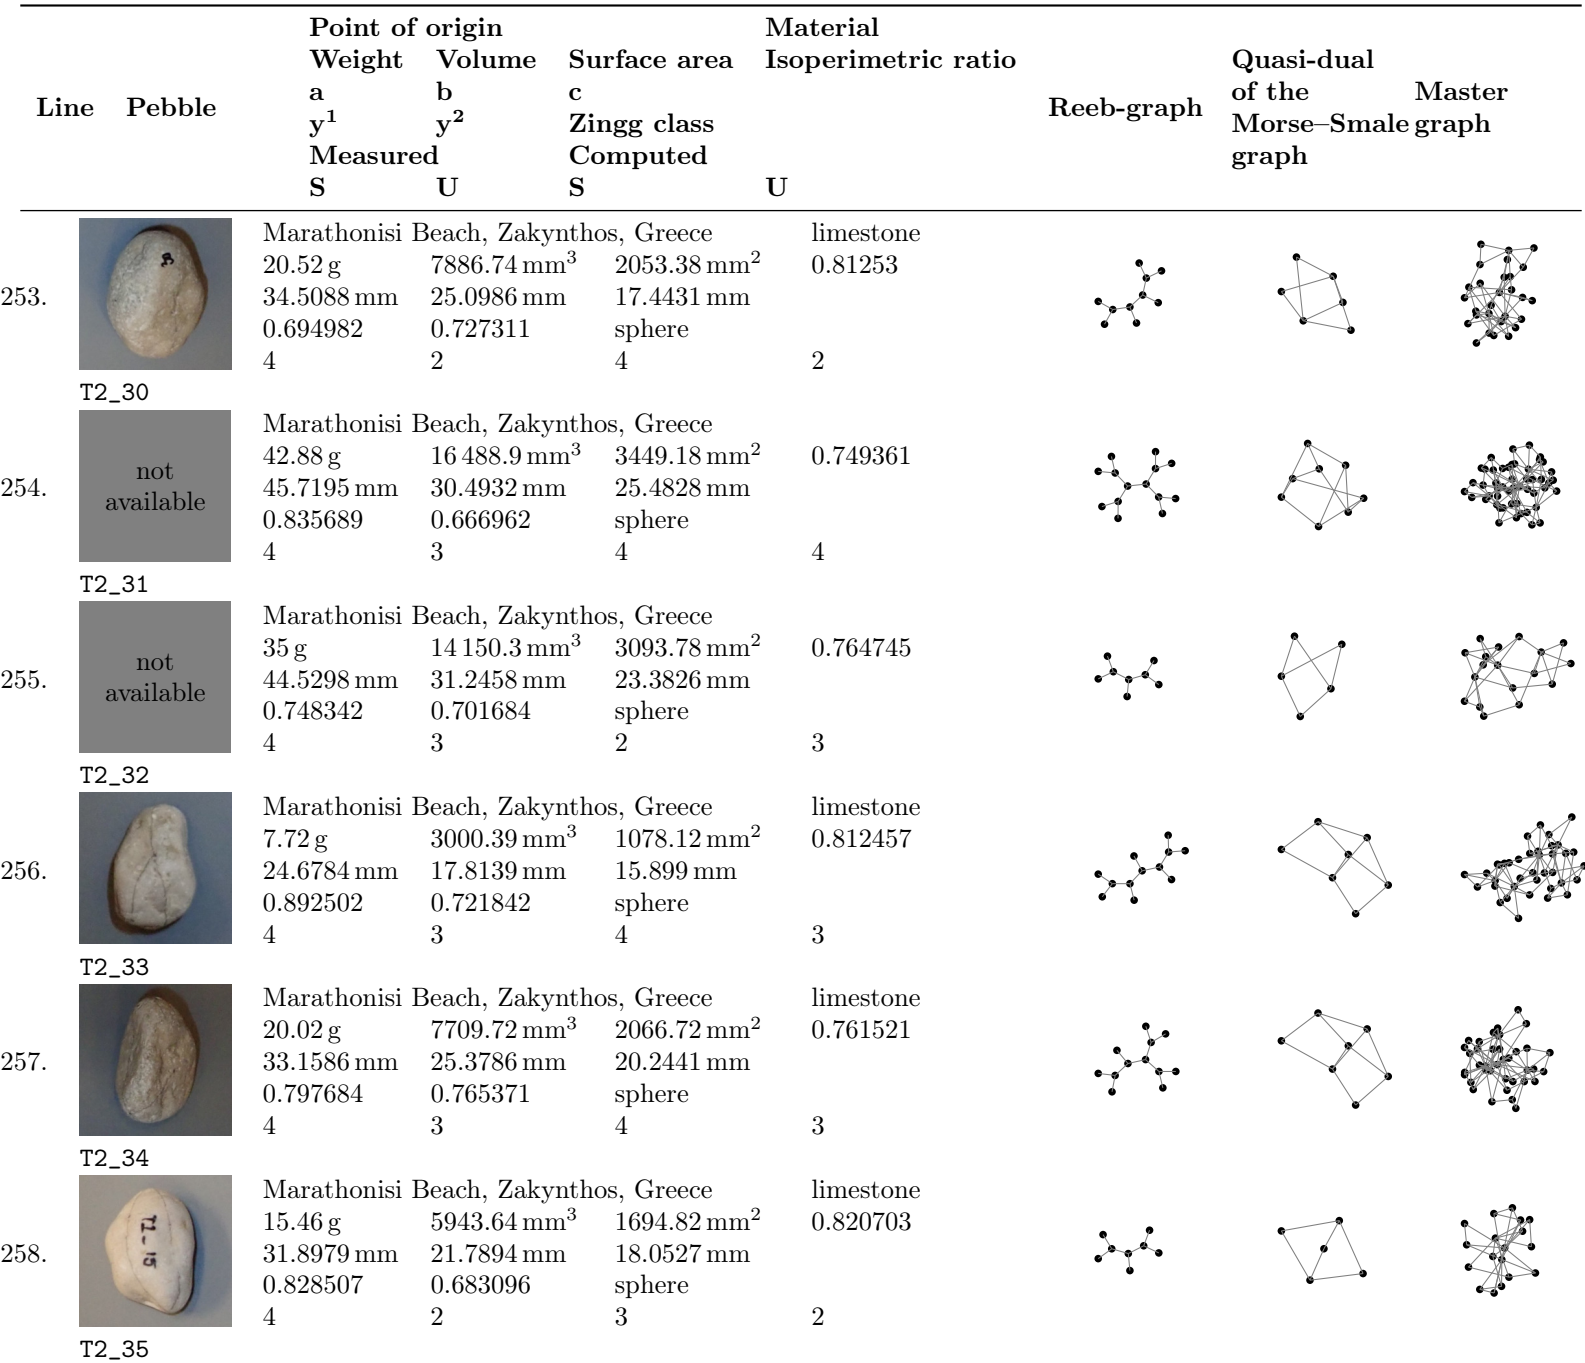   | Marathonisi Beach, Zakynthos, Greece<br>42.88 g<br>45.7195 mm<br>0.835689<br>4 | 42.88 g<br>16 488.9 mm <sup>3</sup><br>30.4932 mm<br>0.666962<br>3 | 3449.18 mm <sup>2</sup><br>25.4828 mm<br>sphere<br>4 | 0.749361<br><br>4                    | 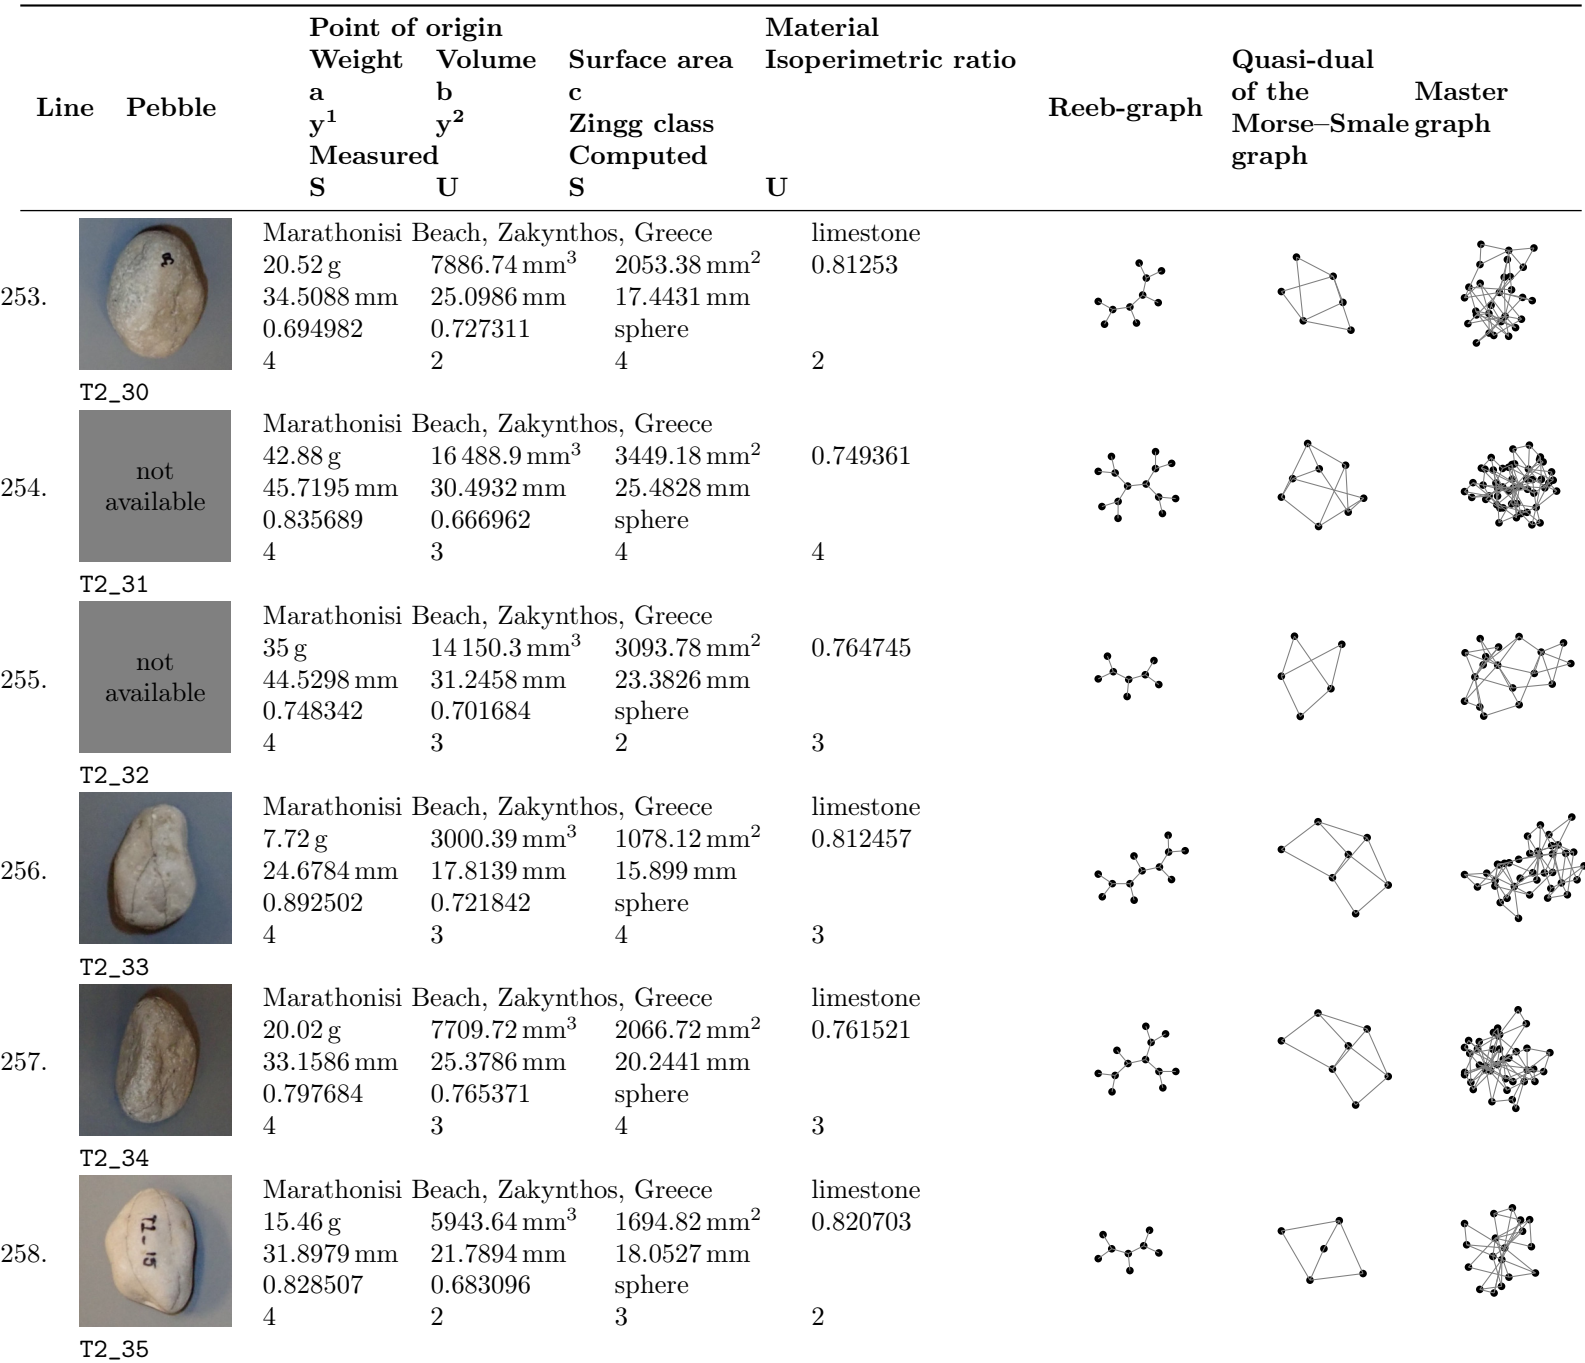   | 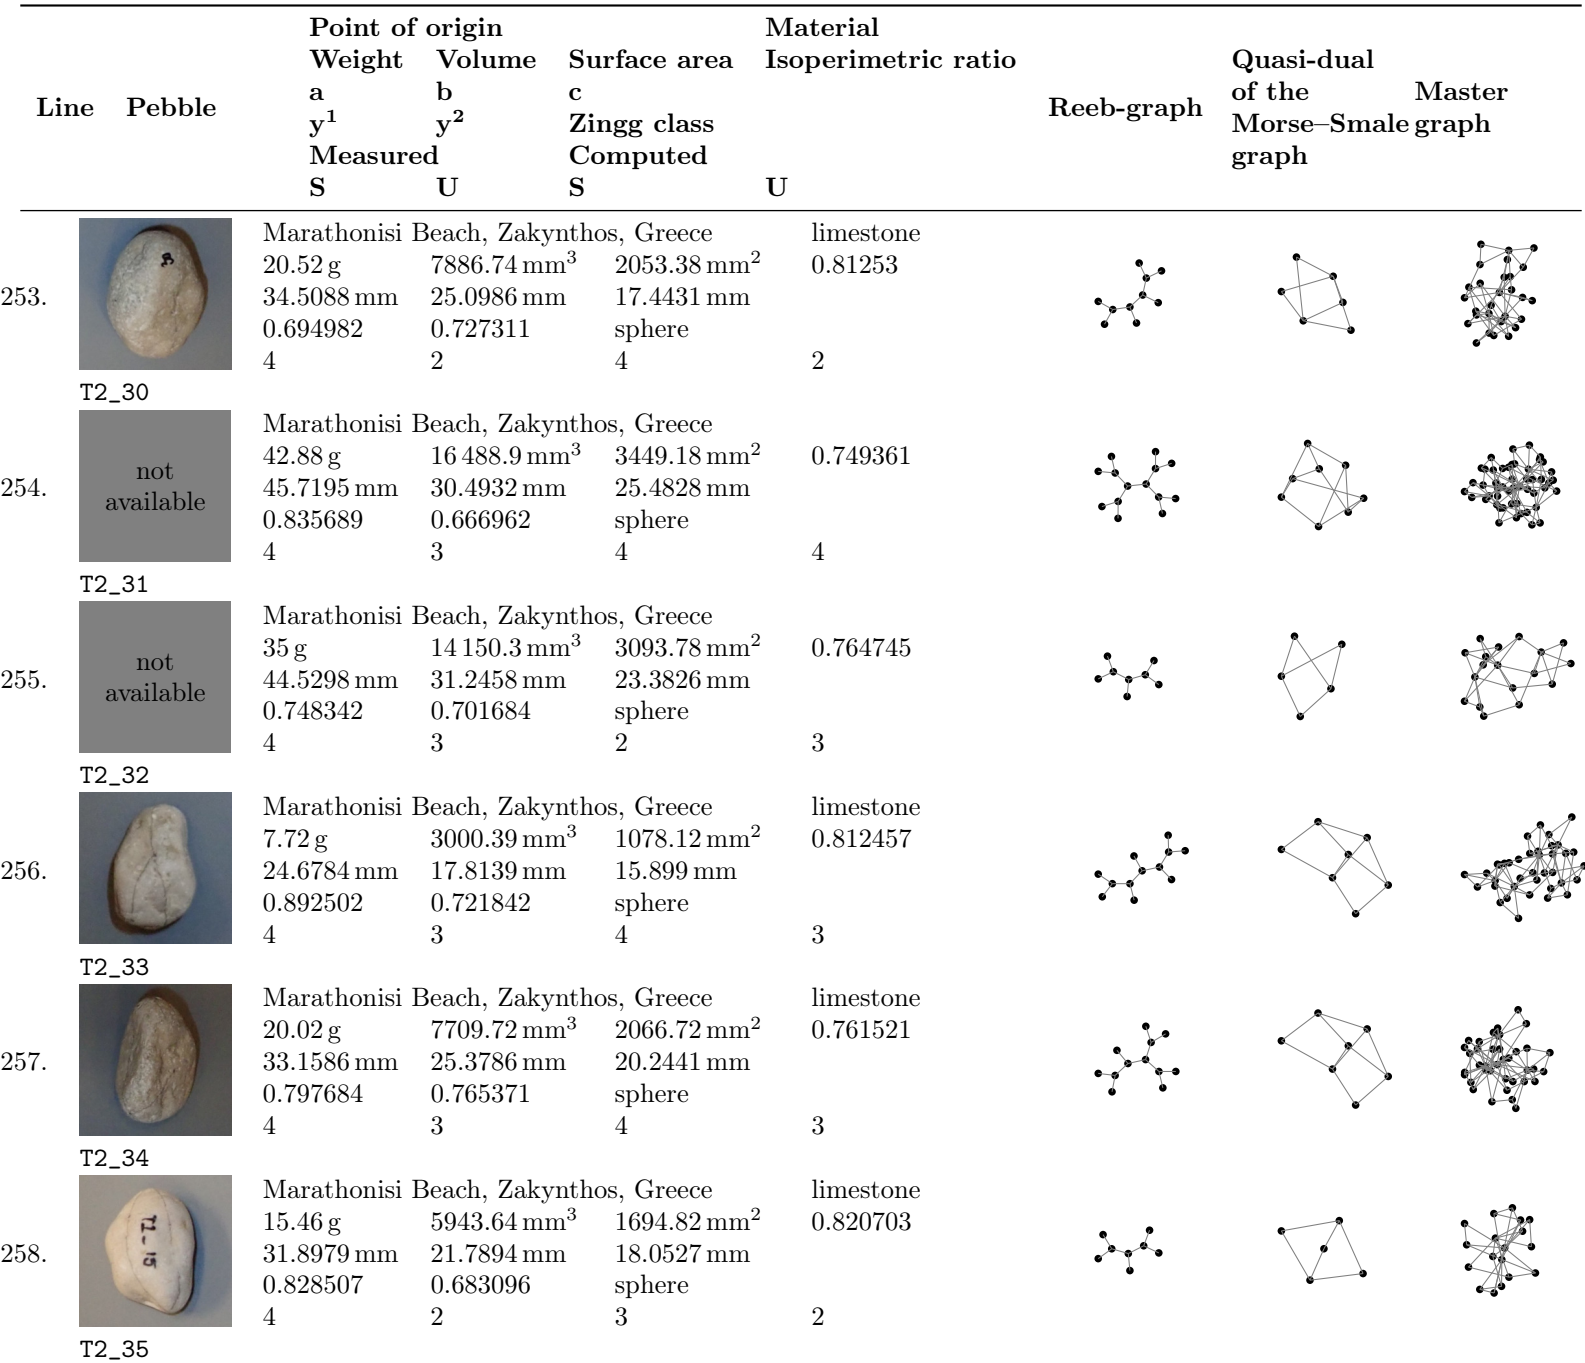   | 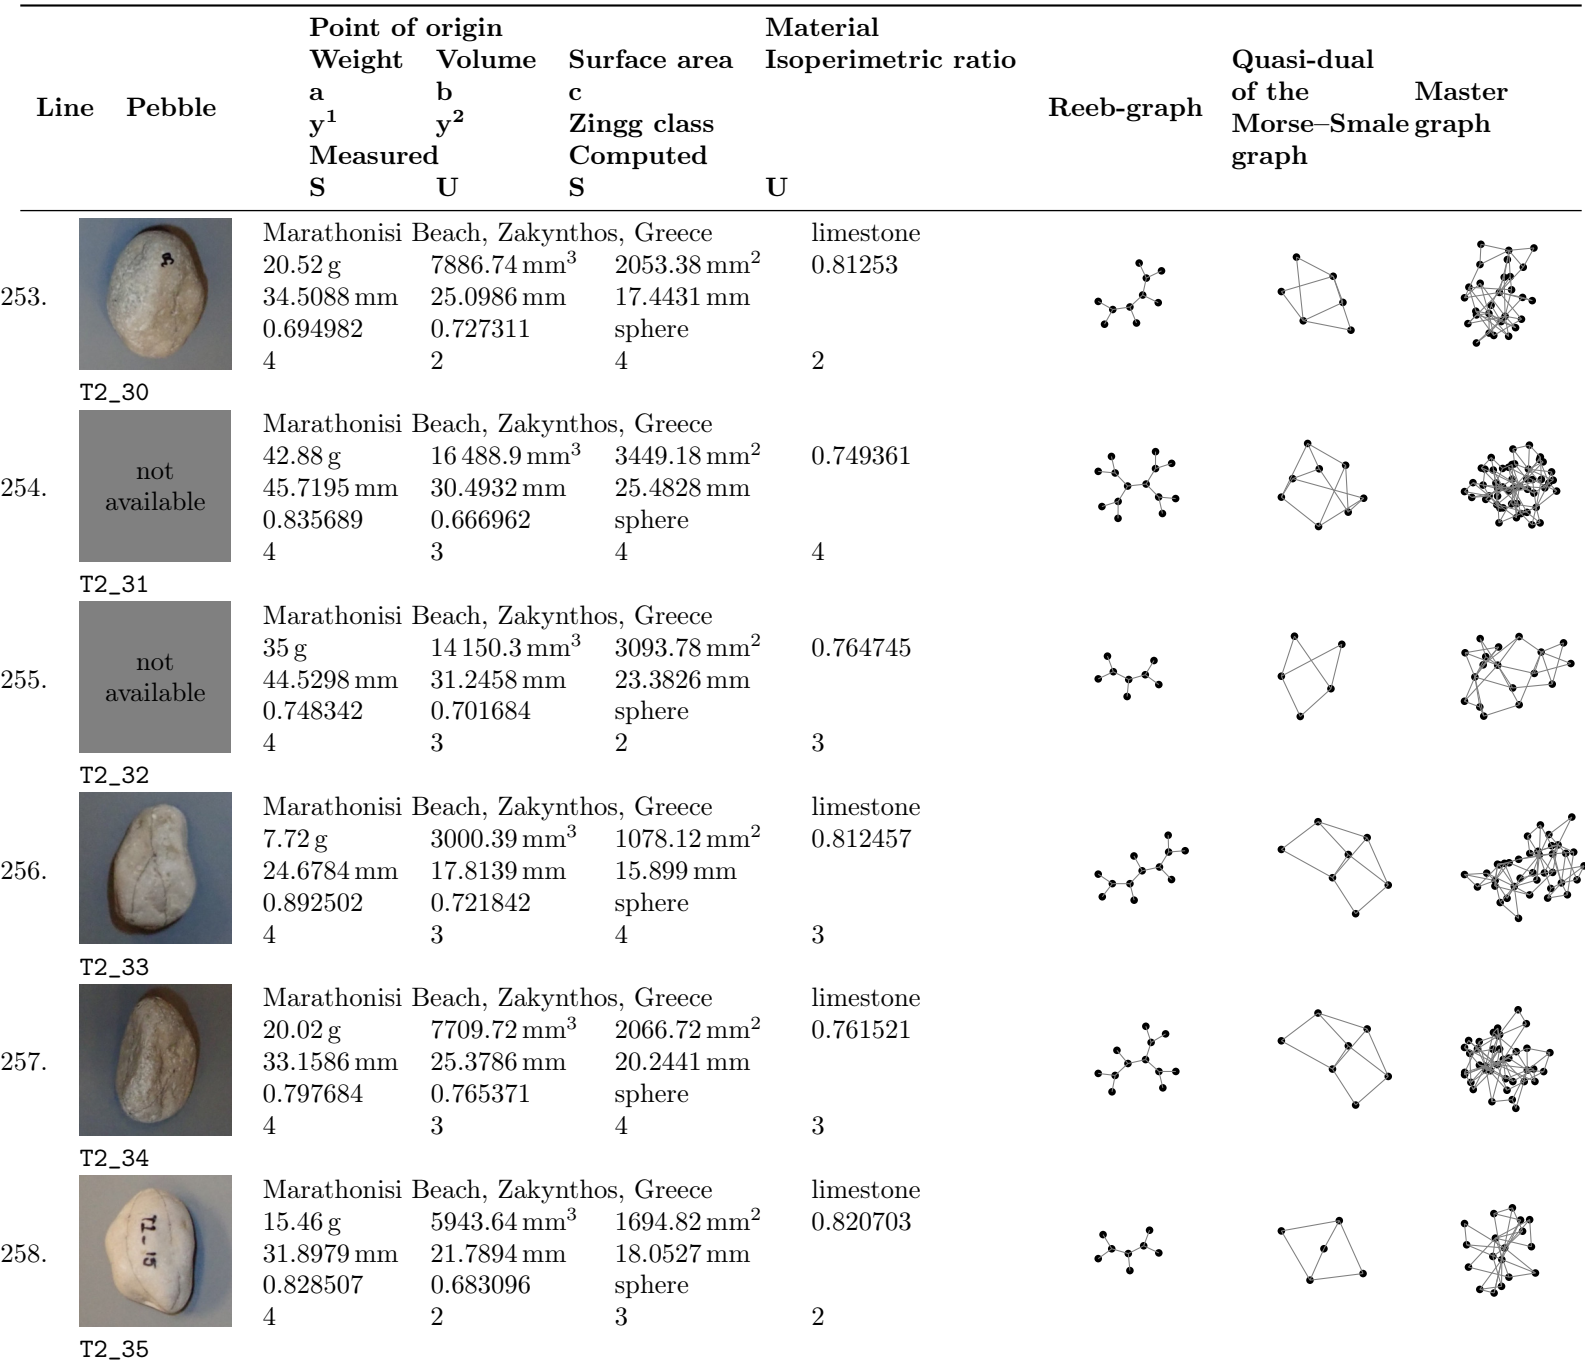   |
|      | T2_31                                                                               |                                                                                |                                                                    |                                                      |                                      |                                                                                       |                                                                                       |                                                                                       |
| 255. | 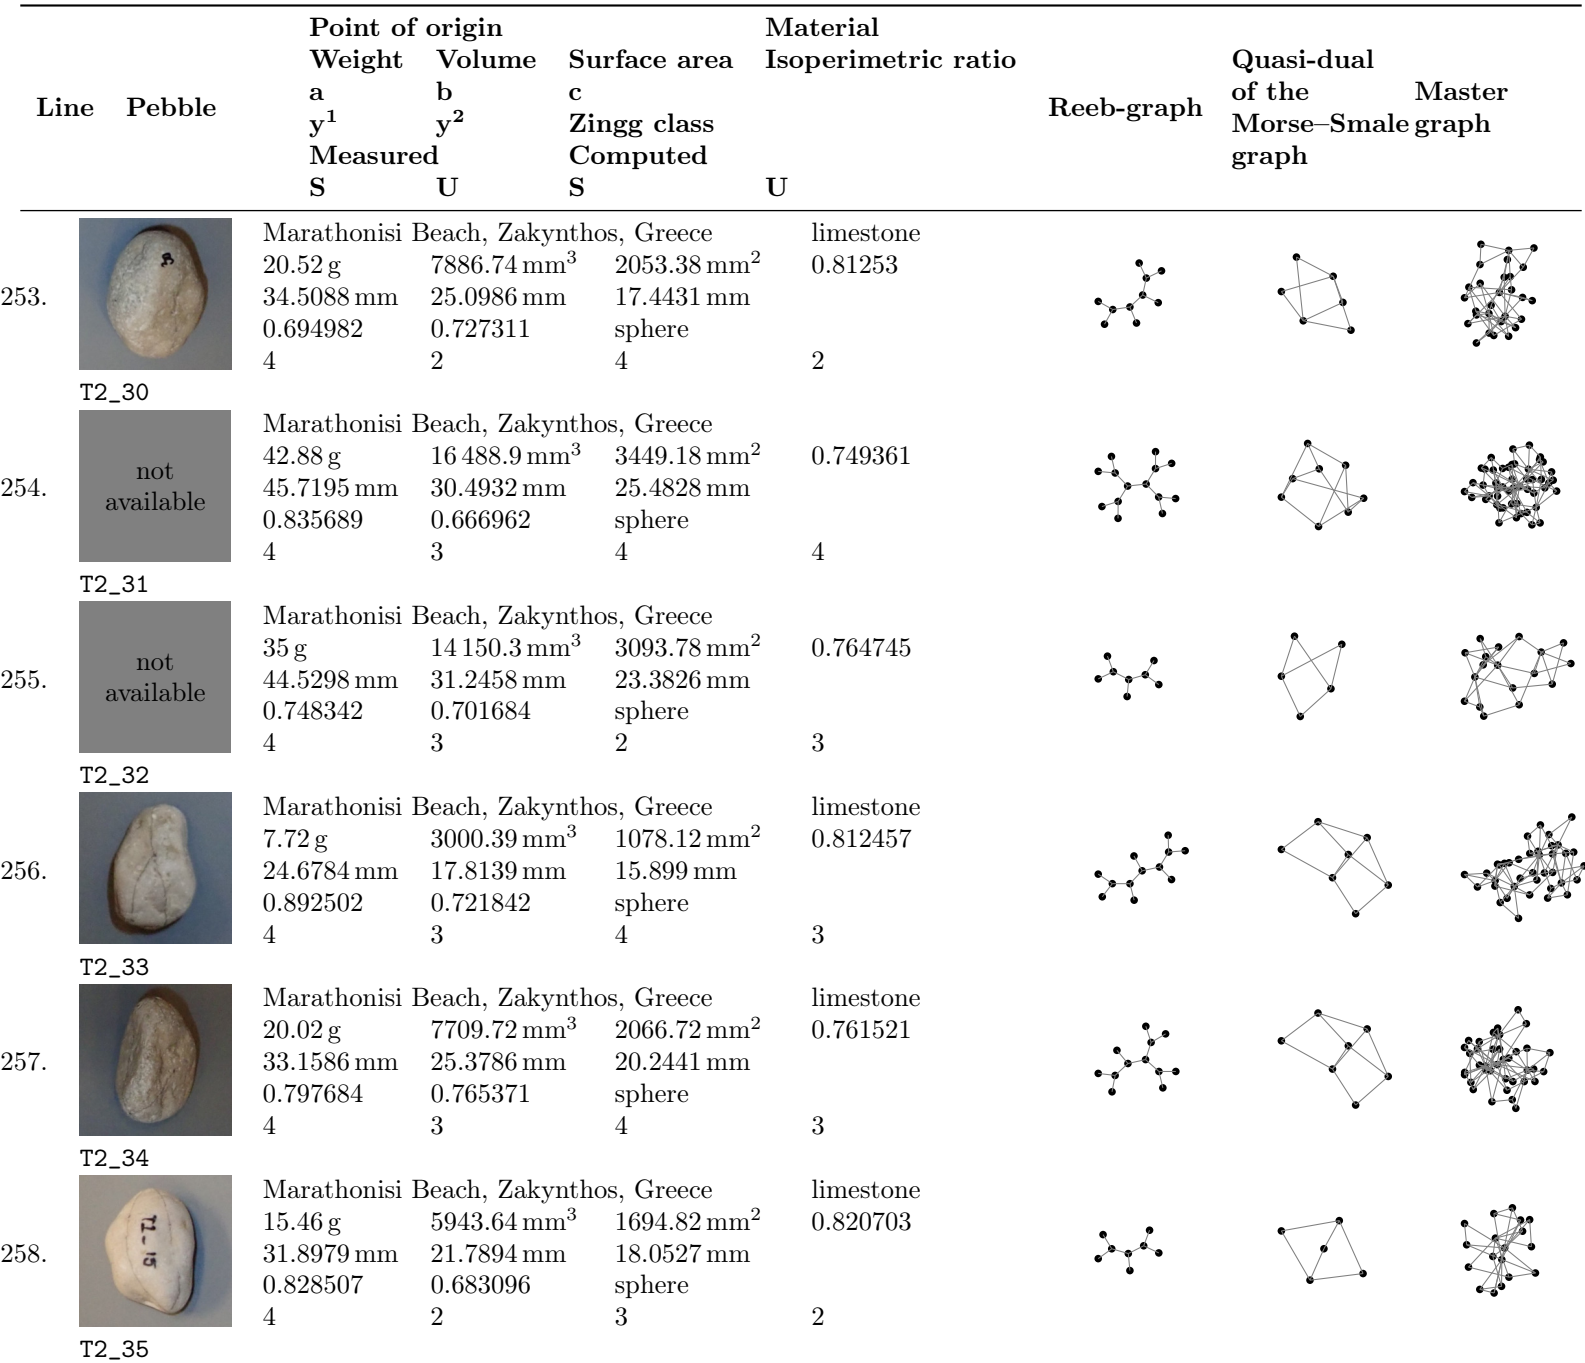   | Marathonisi Beach, Zakynthos, Greece<br>35 g<br>44.5298 mm<br>0.748342<br>4    | 35 g<br>14 150.3 mm <sup>3</sup><br>31.2458 mm<br>0.701684<br>3    | 3093.78 mm <sup>2</sup><br>23.3826 mm<br>sphere<br>2 | 0.764745<br><br>3                    | 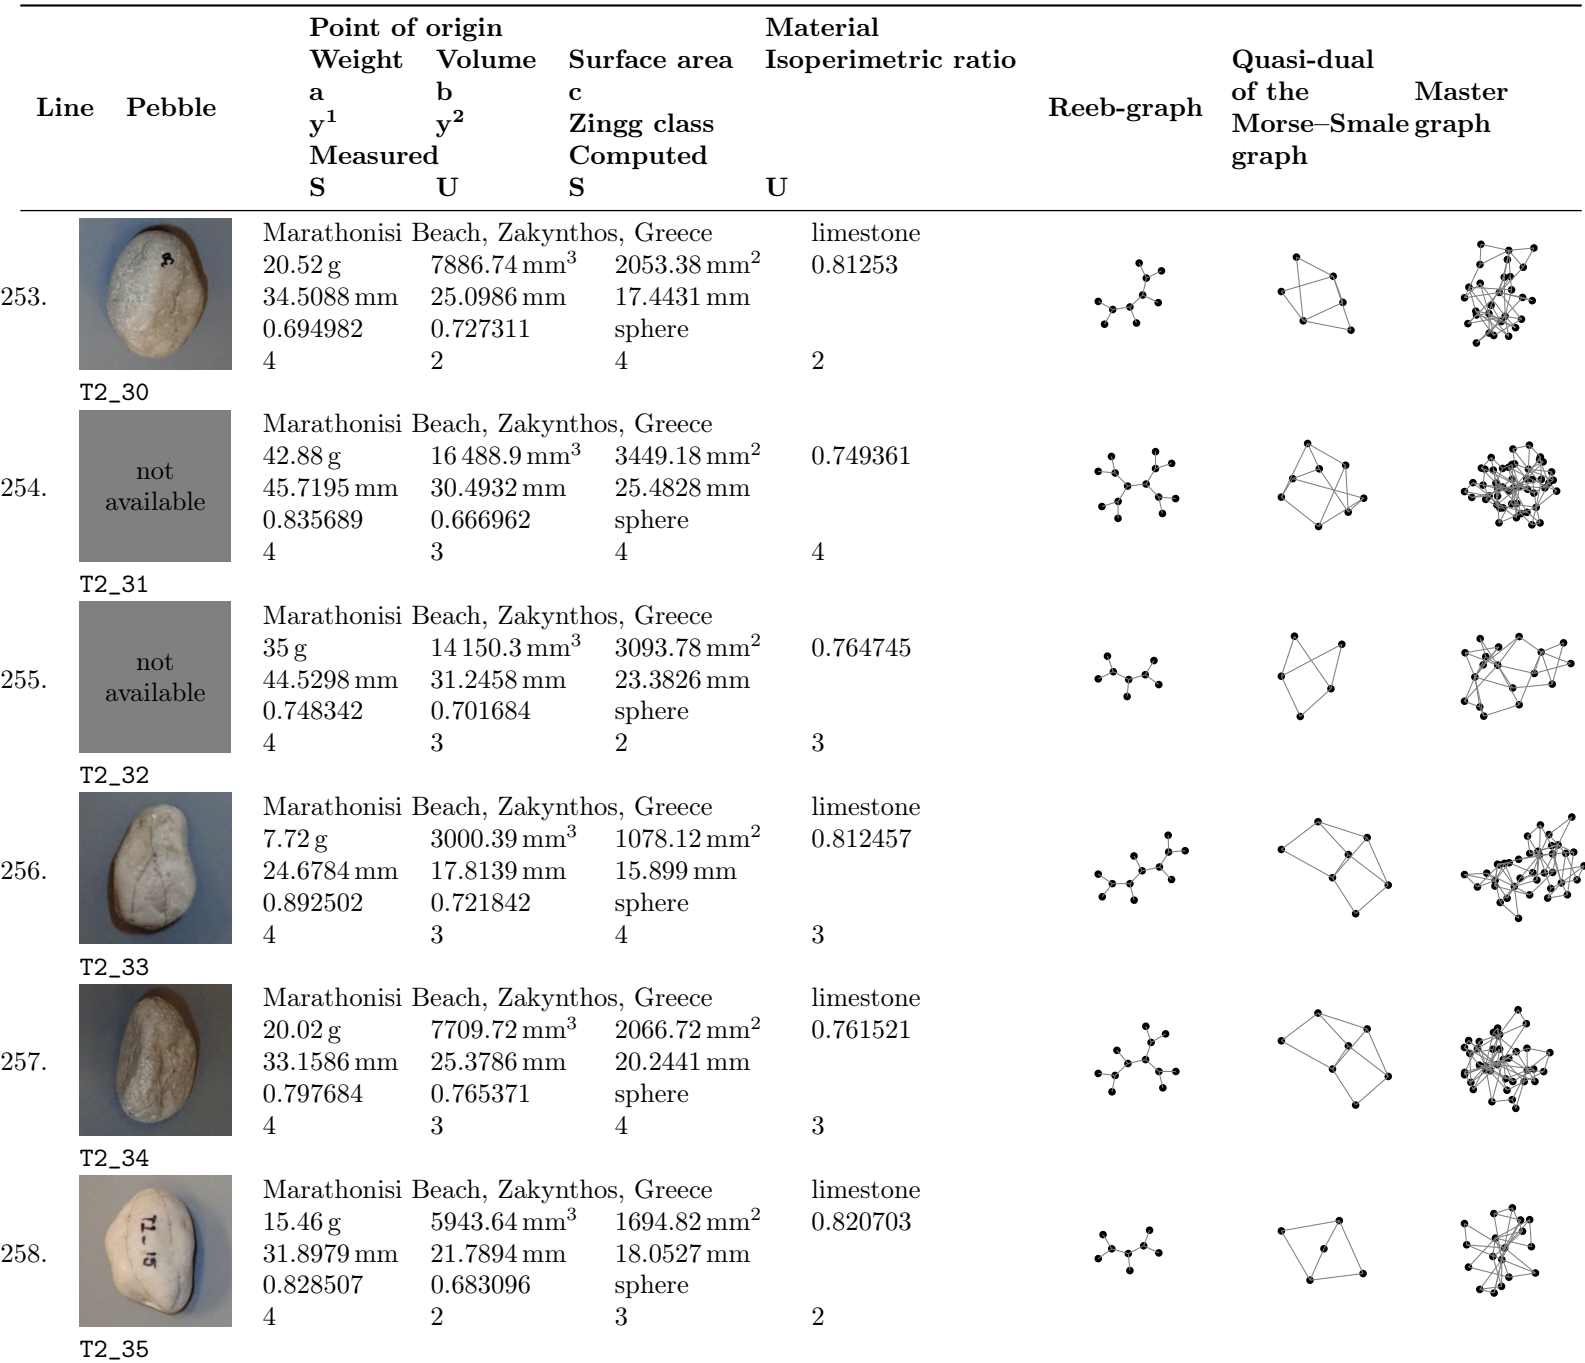   | 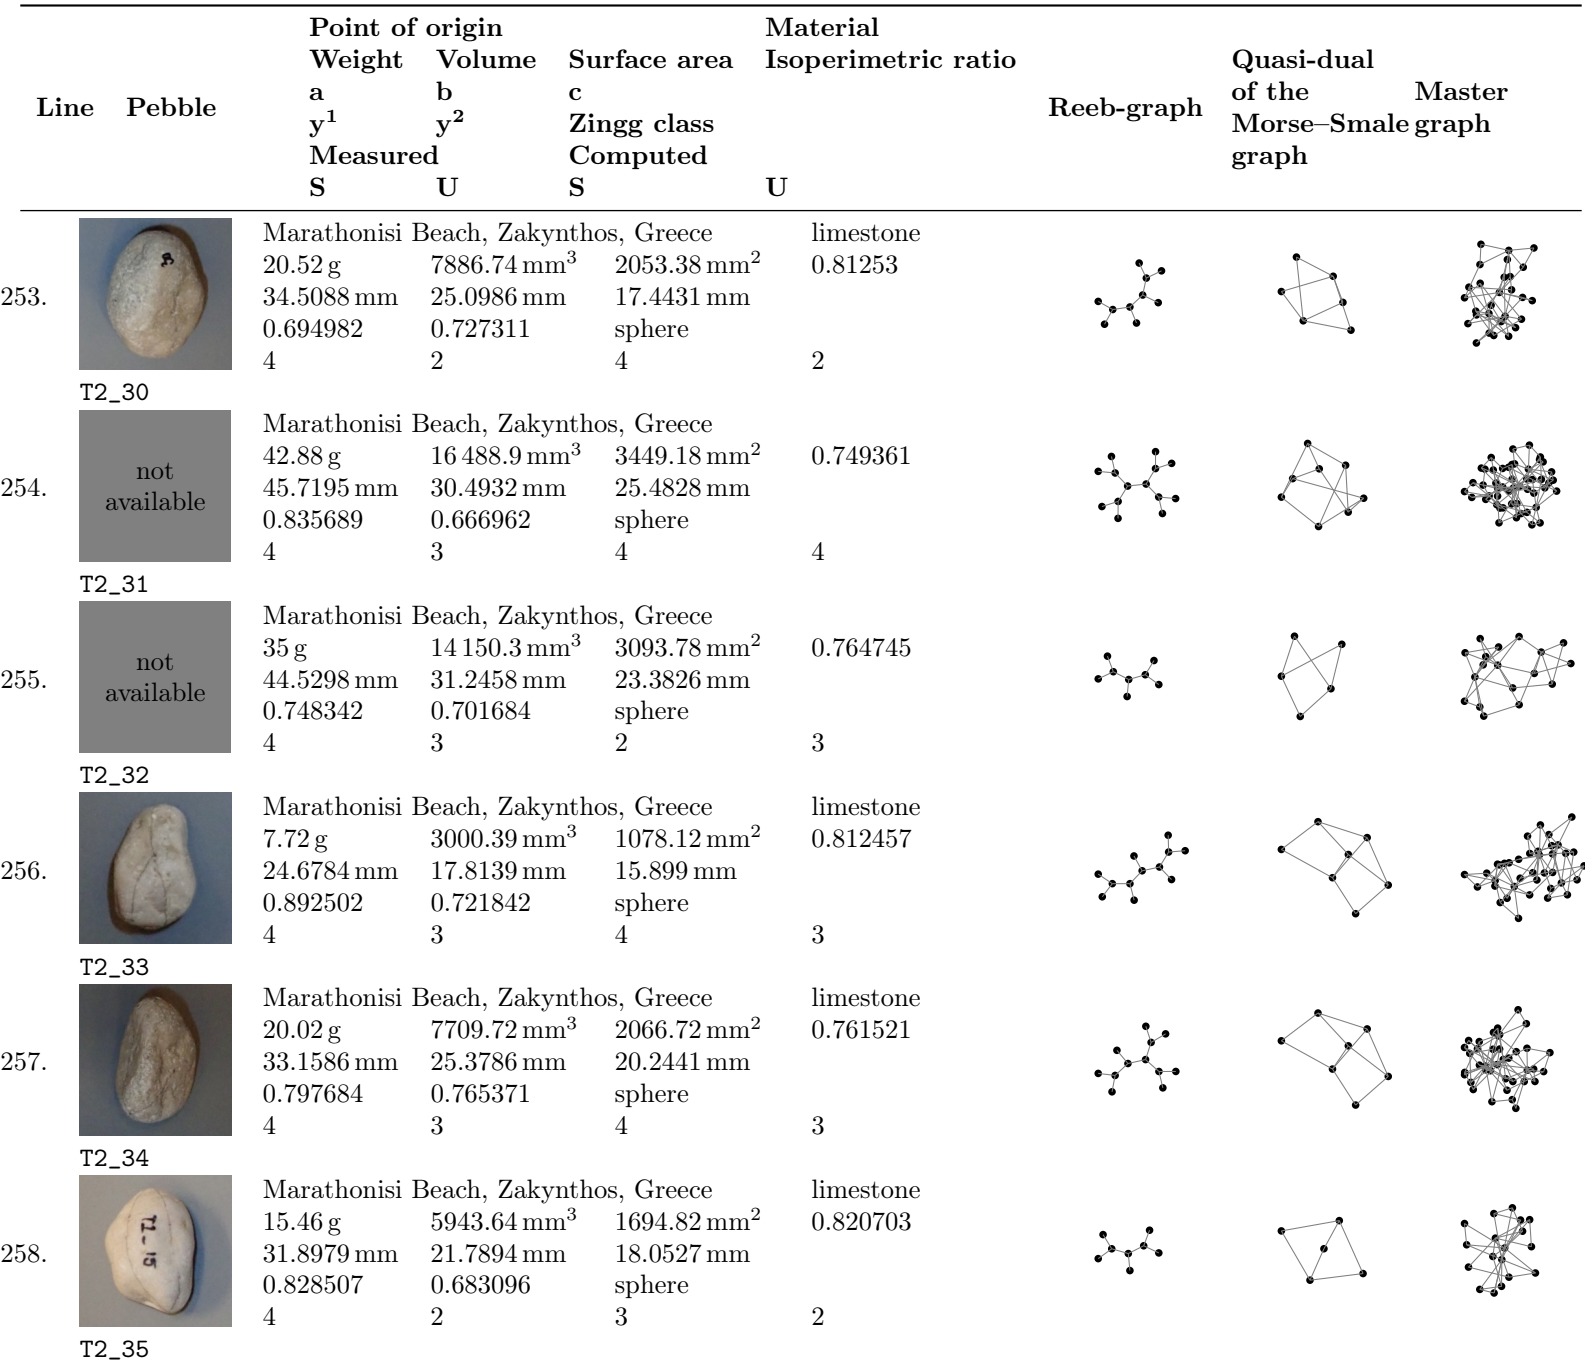   | 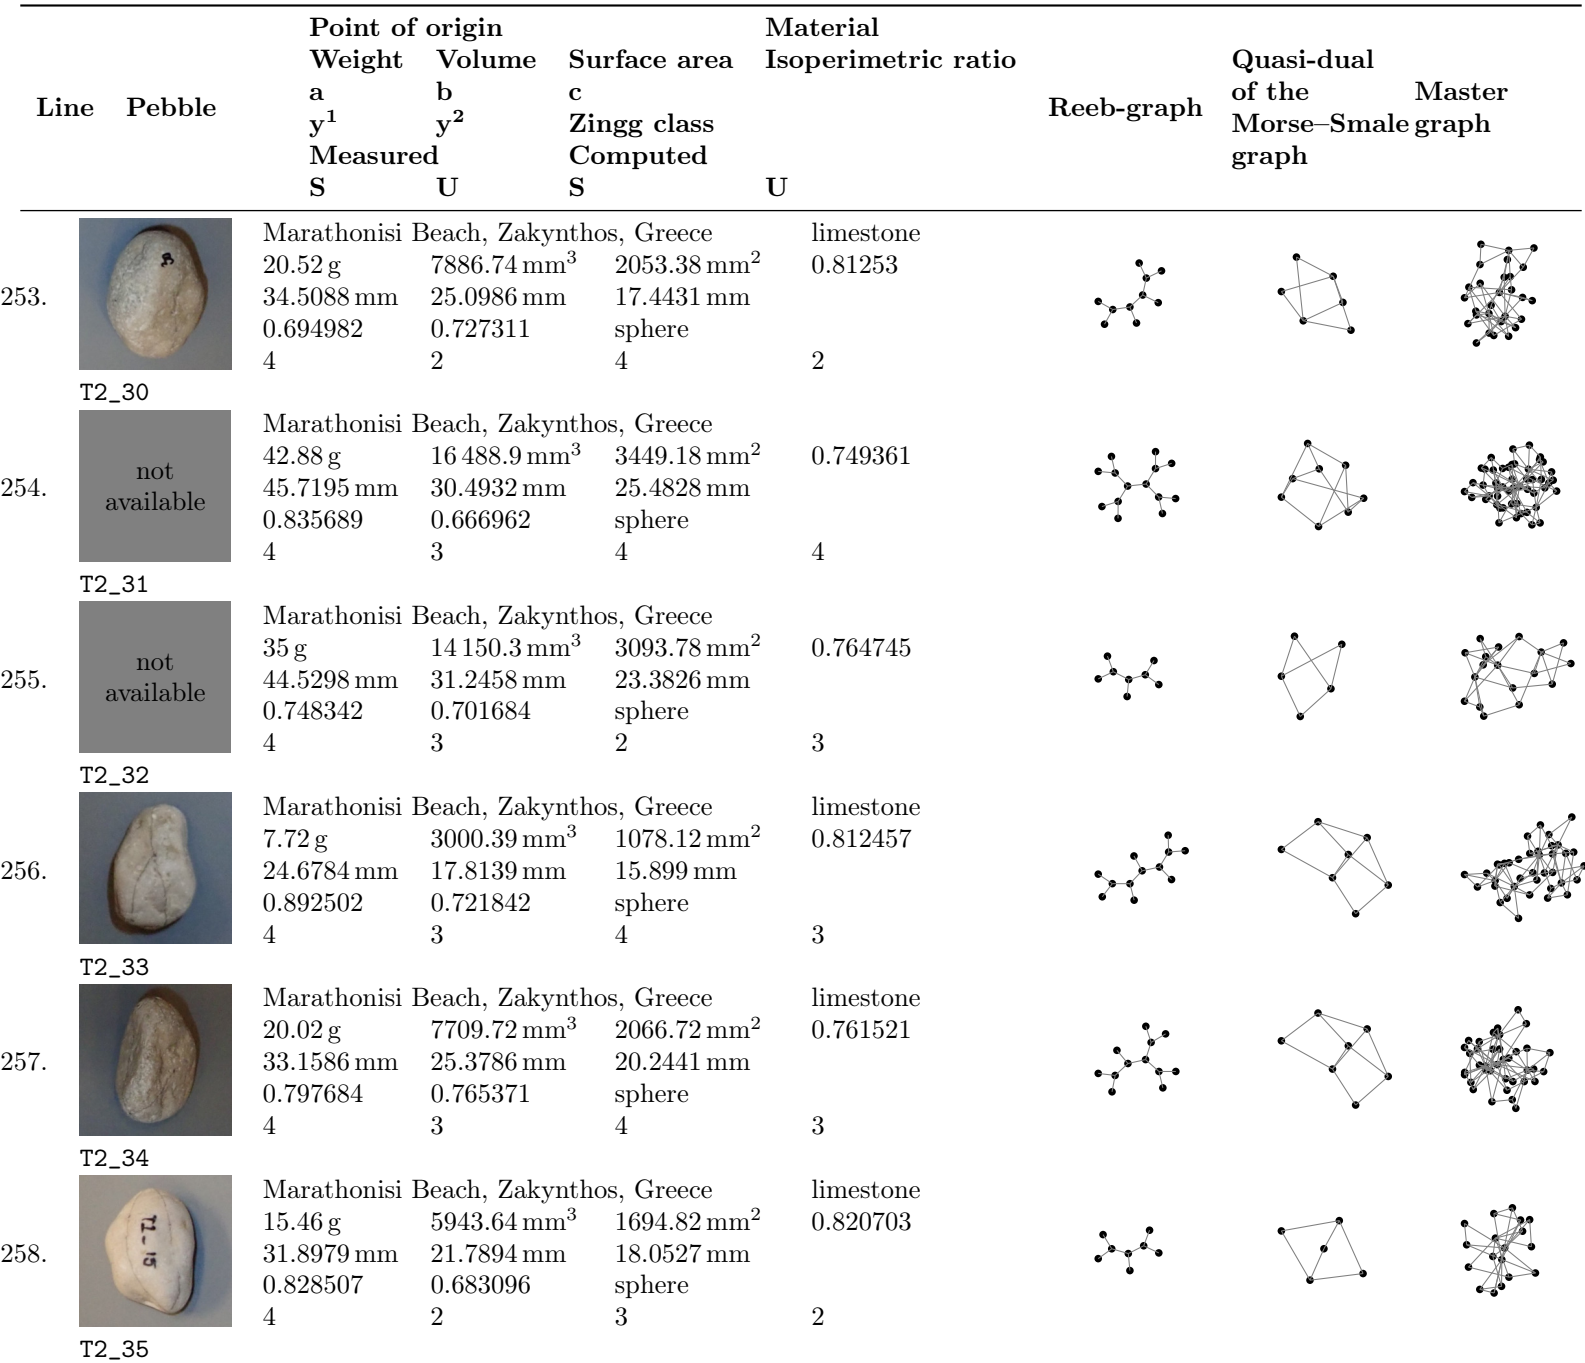   |
|      | T2_32                                                                               |                                                                                |                                                                    |                                                      |                                      |                                                                                       |                                                                                       |                                                                                       |
| 256. | 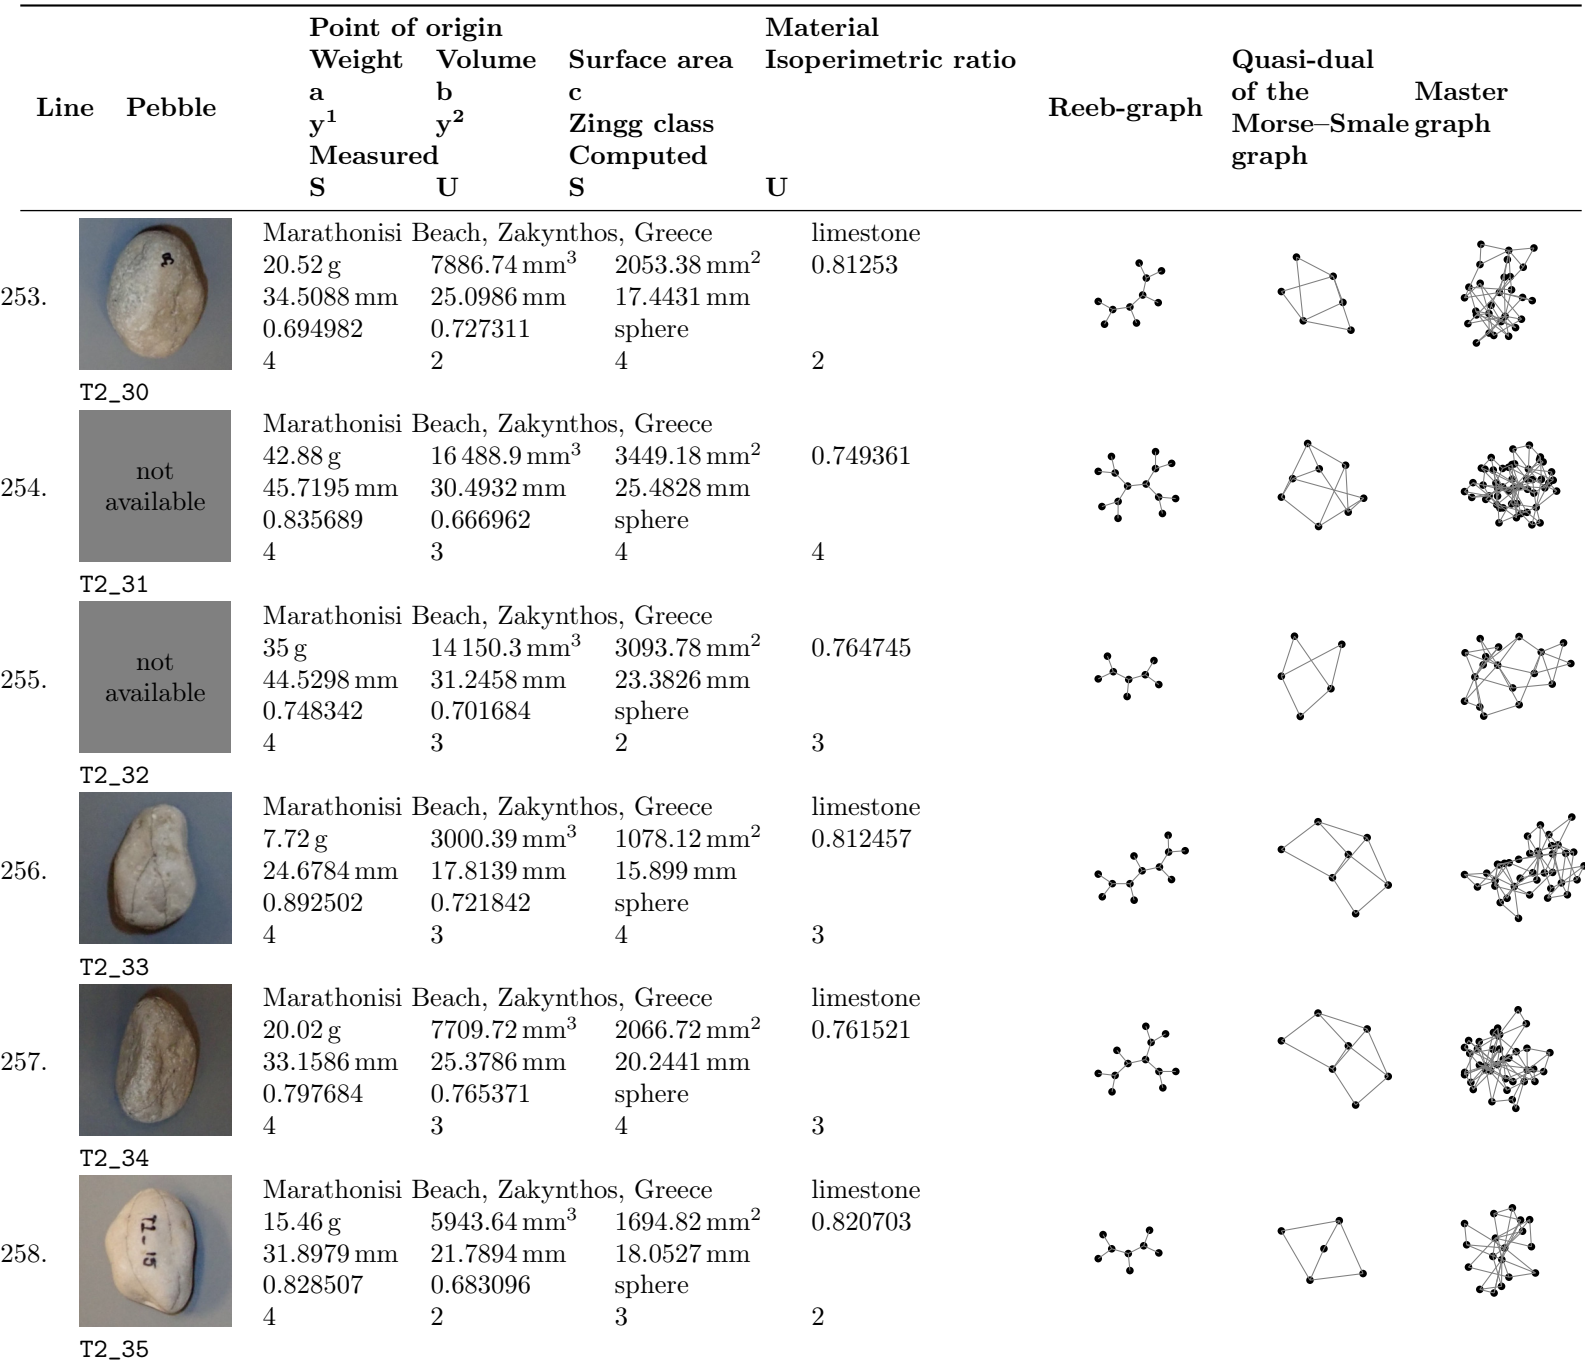  | Marathonisi Beach, Zakynthos, Greece<br>7.72 g<br>24.6784 mm<br>0.892502<br>4  | 7.72 g<br>3000.39 mm <sup>3</sup><br>17.8139 mm<br>0.721842<br>3   | 1078.12 mm <sup>2</sup><br>15.899 mm<br>sphere<br>4  | limestone<br>0.812457<br><br>3       | 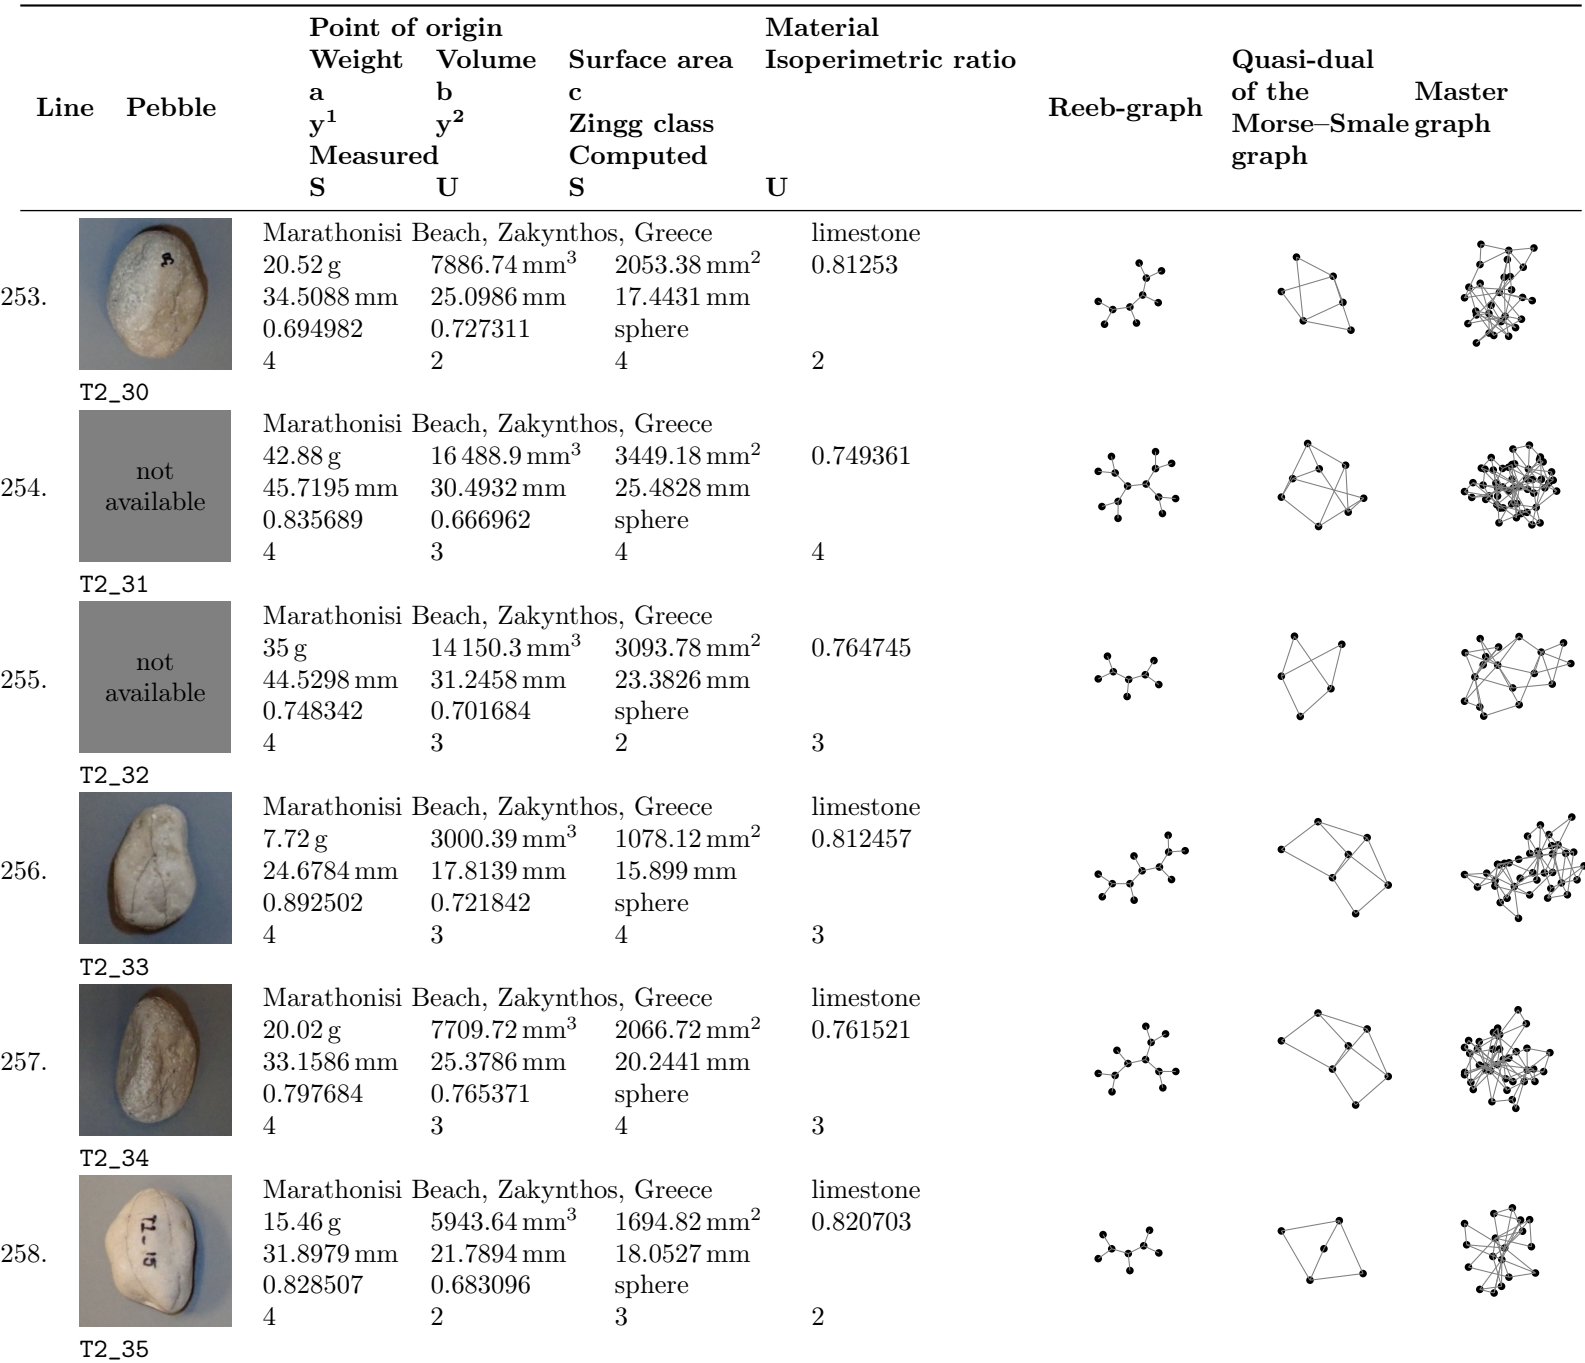  | 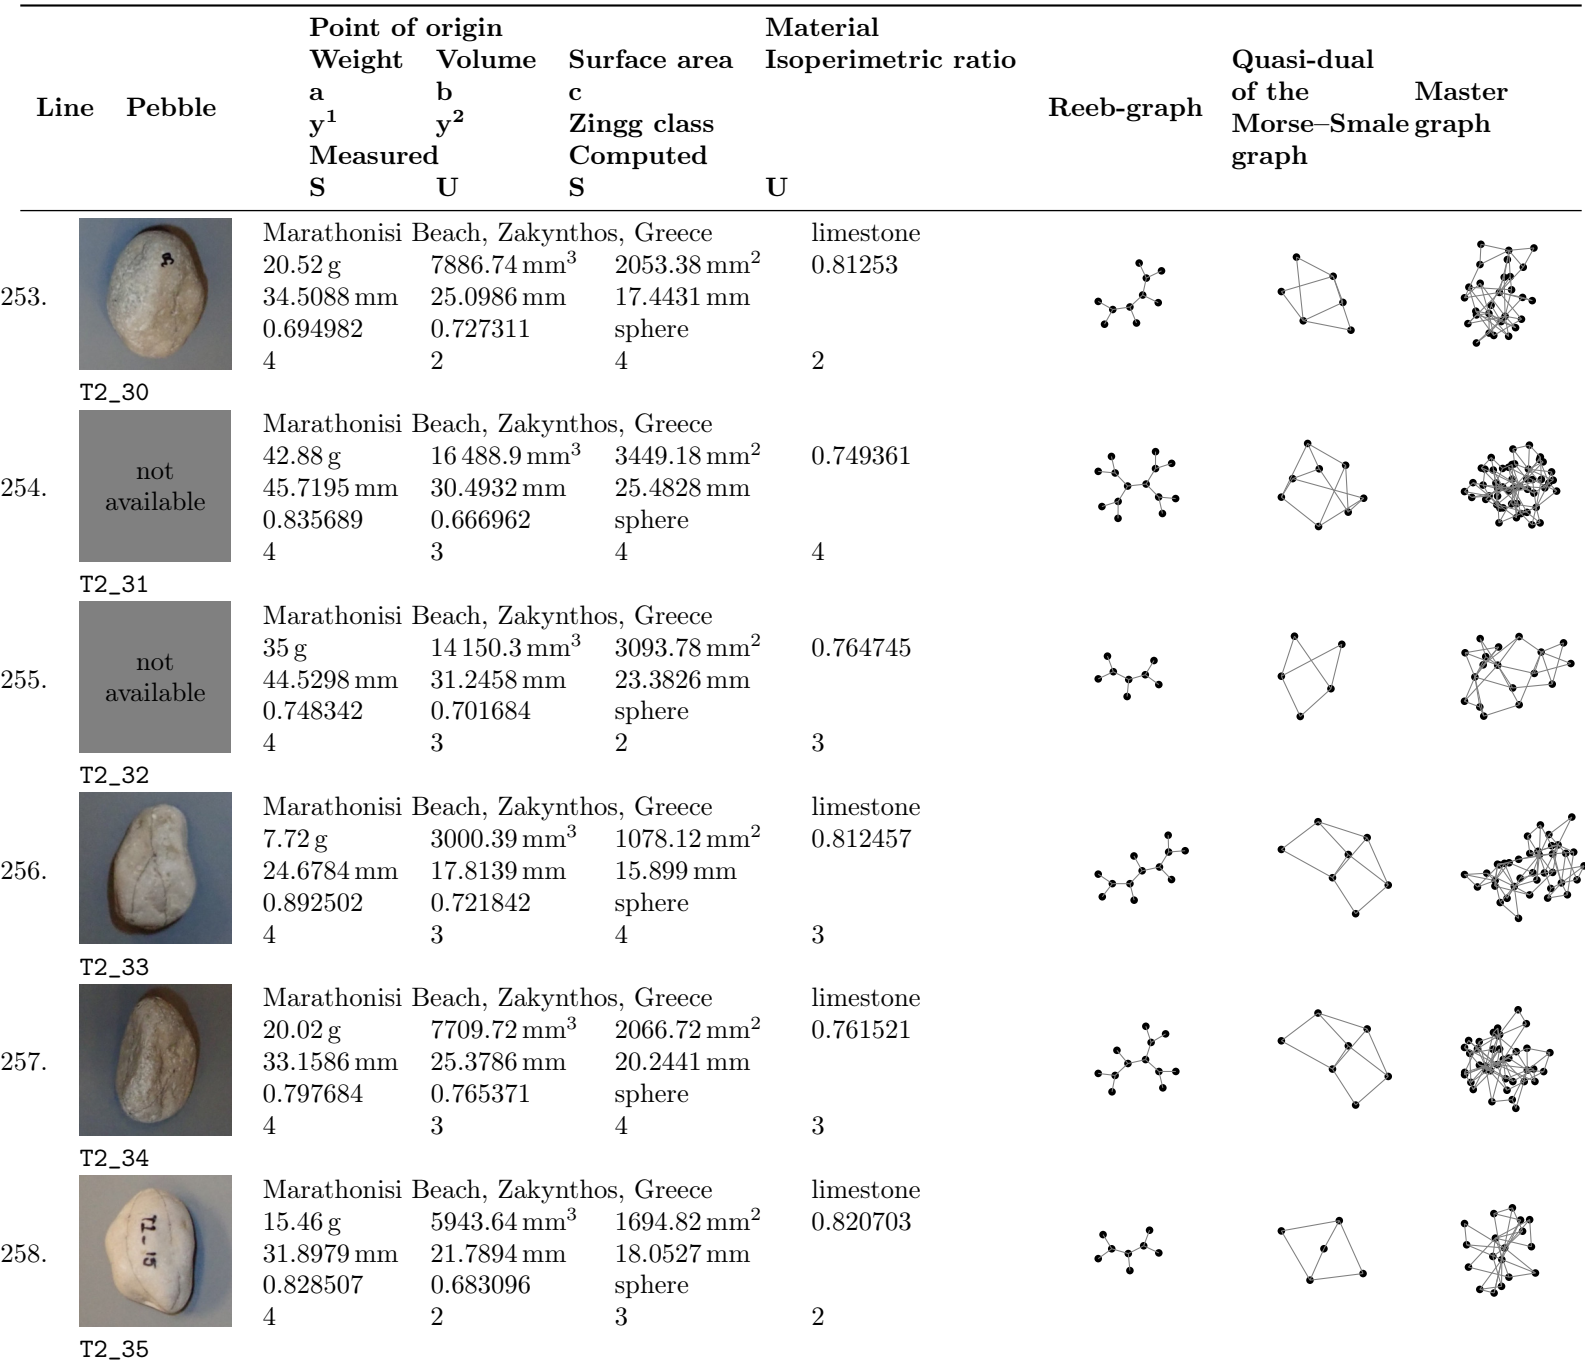  | 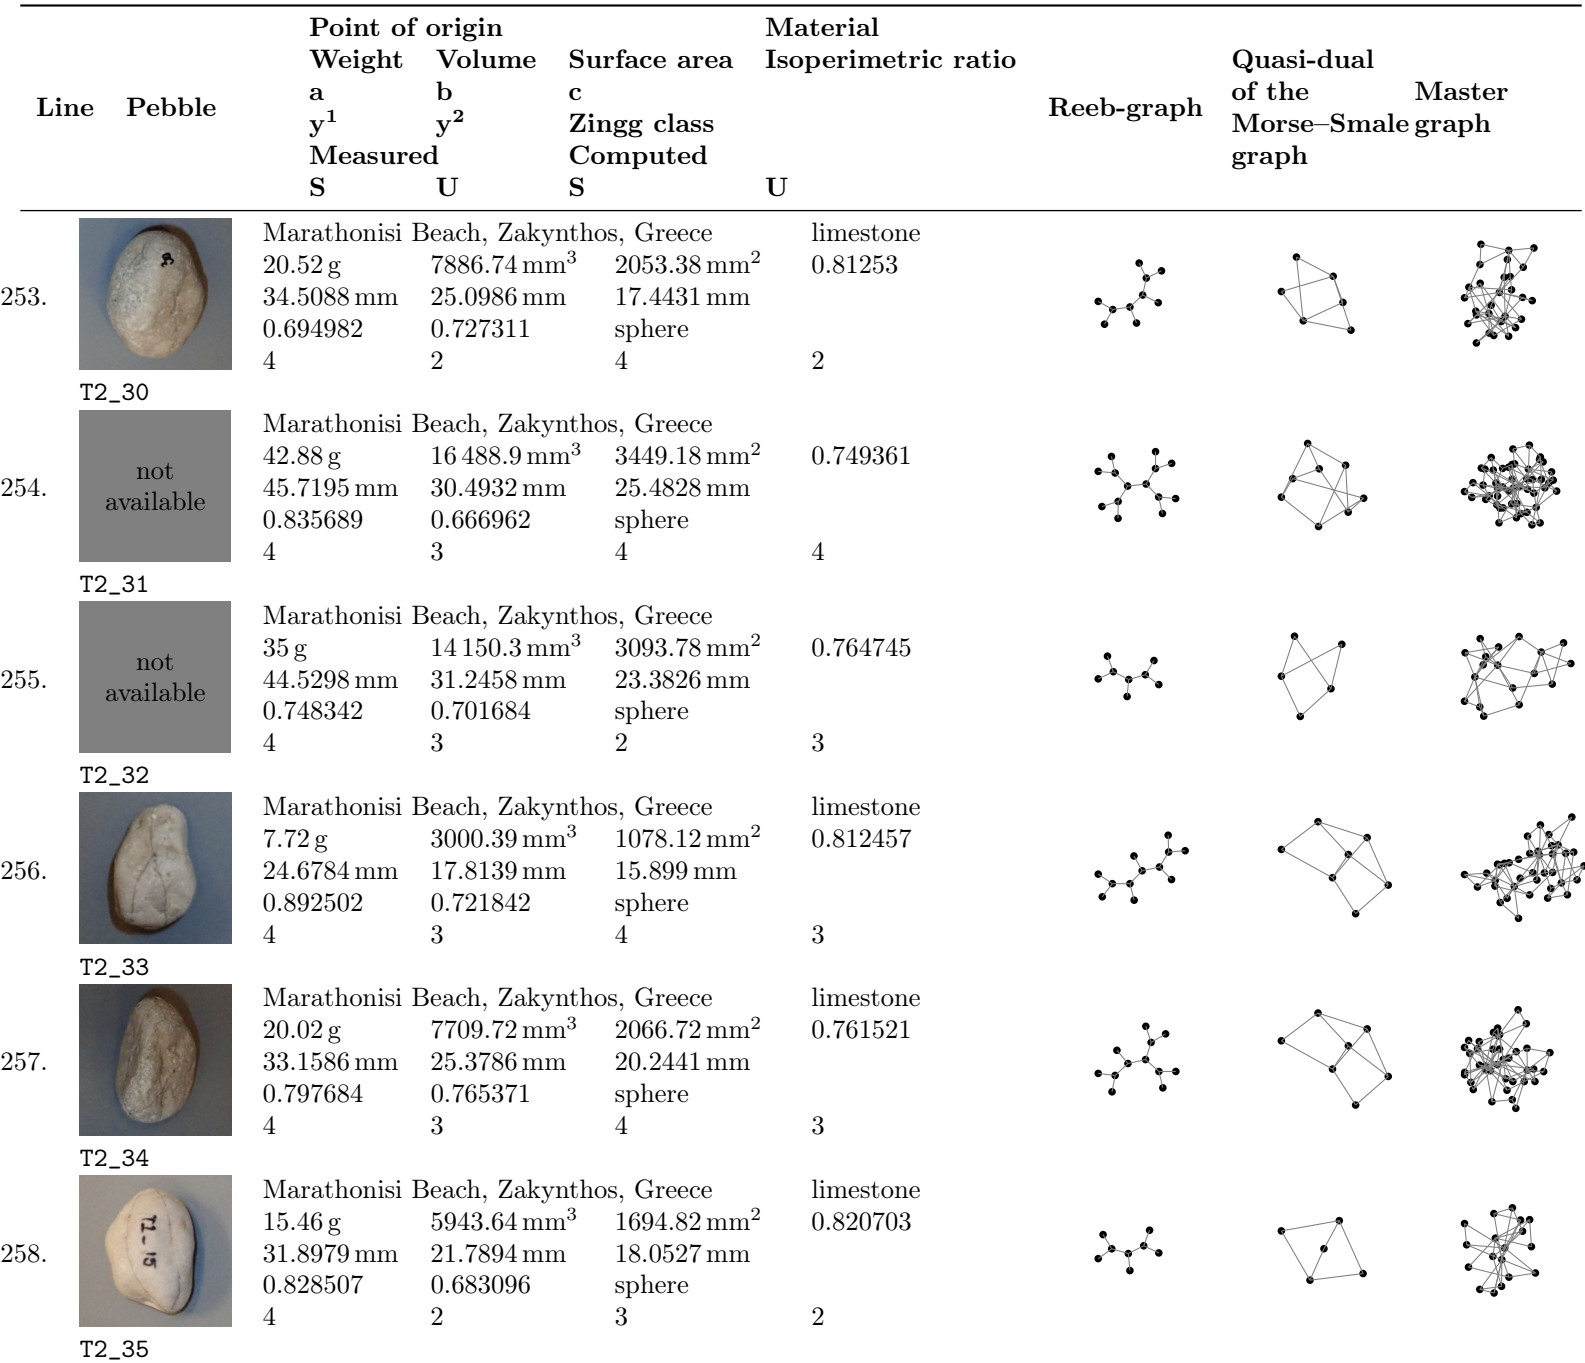  |
|      | T2_33                                                                               |                                                                                |                                                                    |                                                      |                                      |                                                                                       |                                                                                       |                                                                                       |
| 257. | 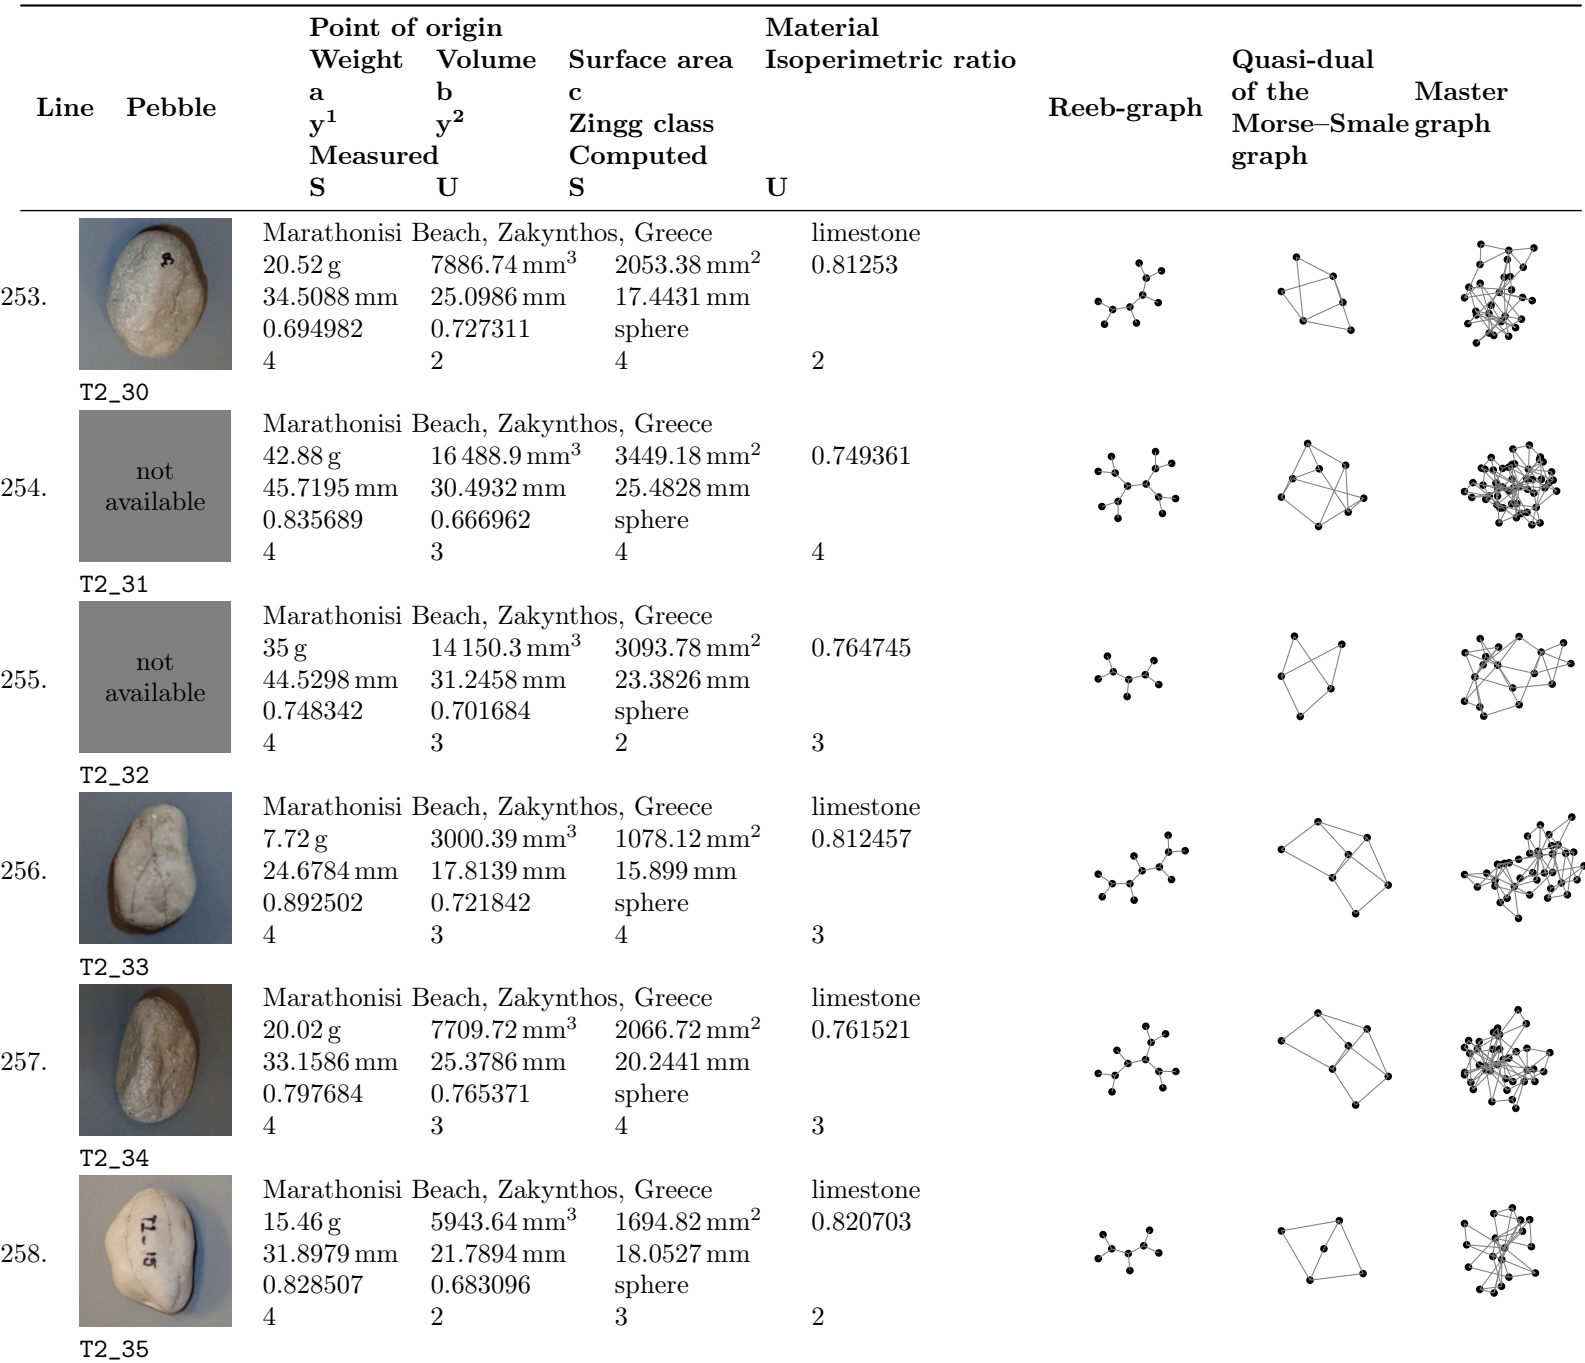 | Marathonisi Beach, Zakynthos, Greece<br>20.02 g<br>33.1586 mm<br>0.797684<br>4 | 20.02 g<br>7709.72 mm <sup>3</sup><br>25.3786 mm<br>0.765371<br>3  | 2066.72 mm <sup>2</sup><br>20.2441 mm<br>sphere<br>4 | limestone<br>0.761521<br><br>3       | 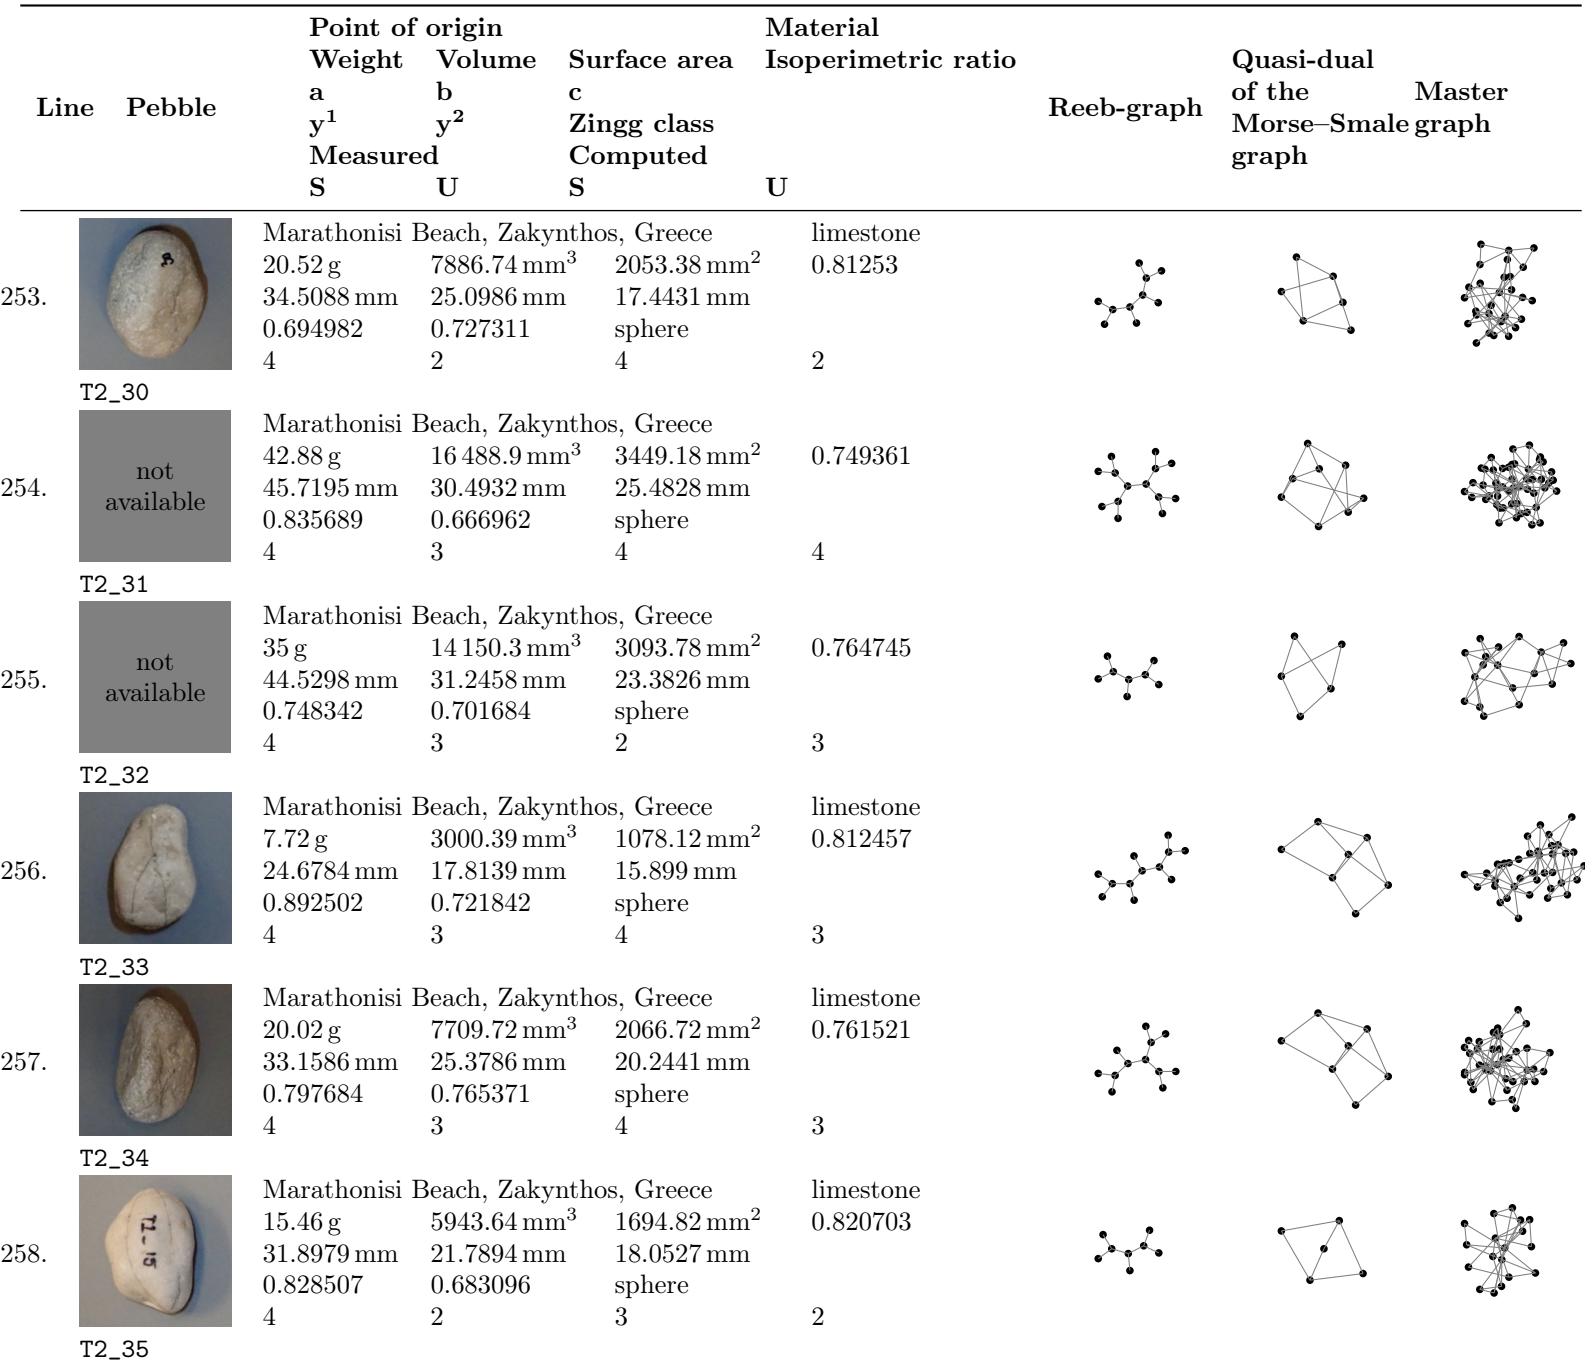 | 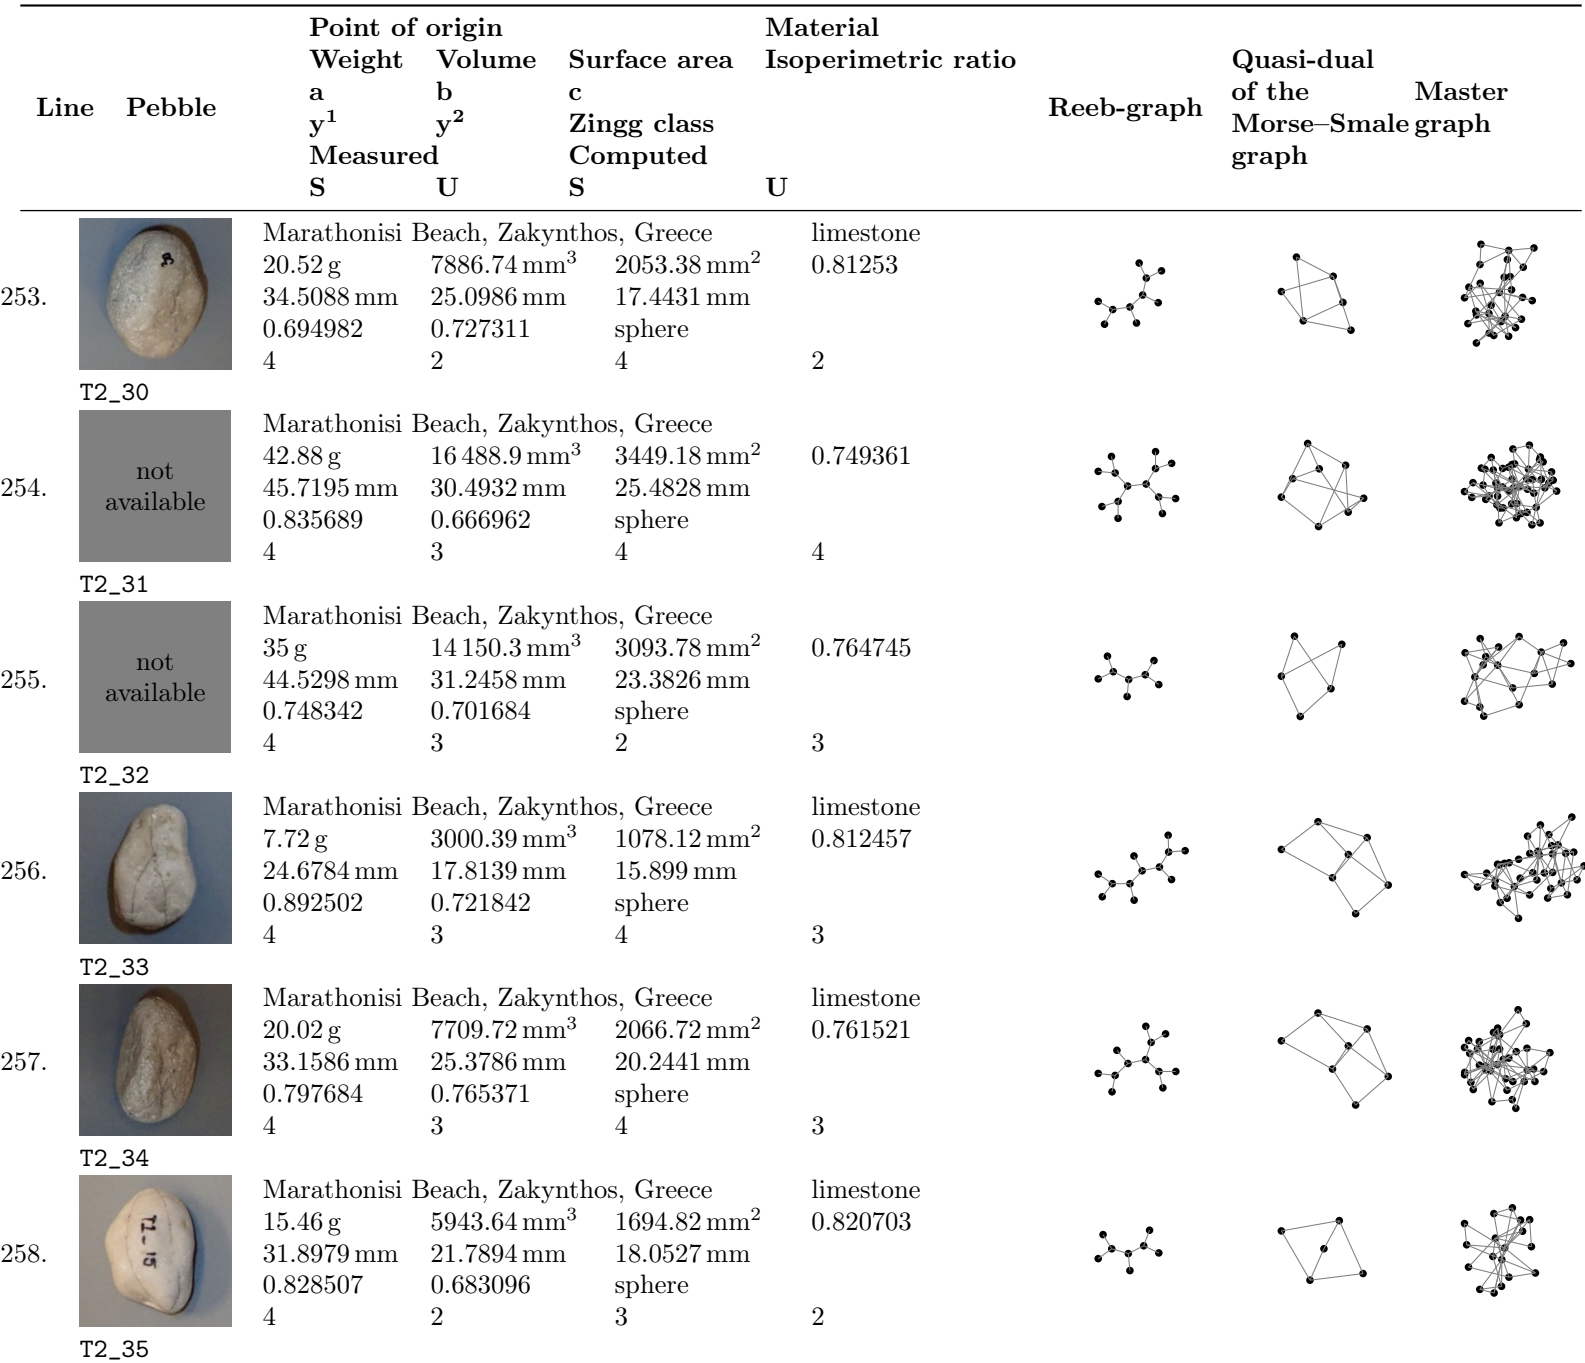 | 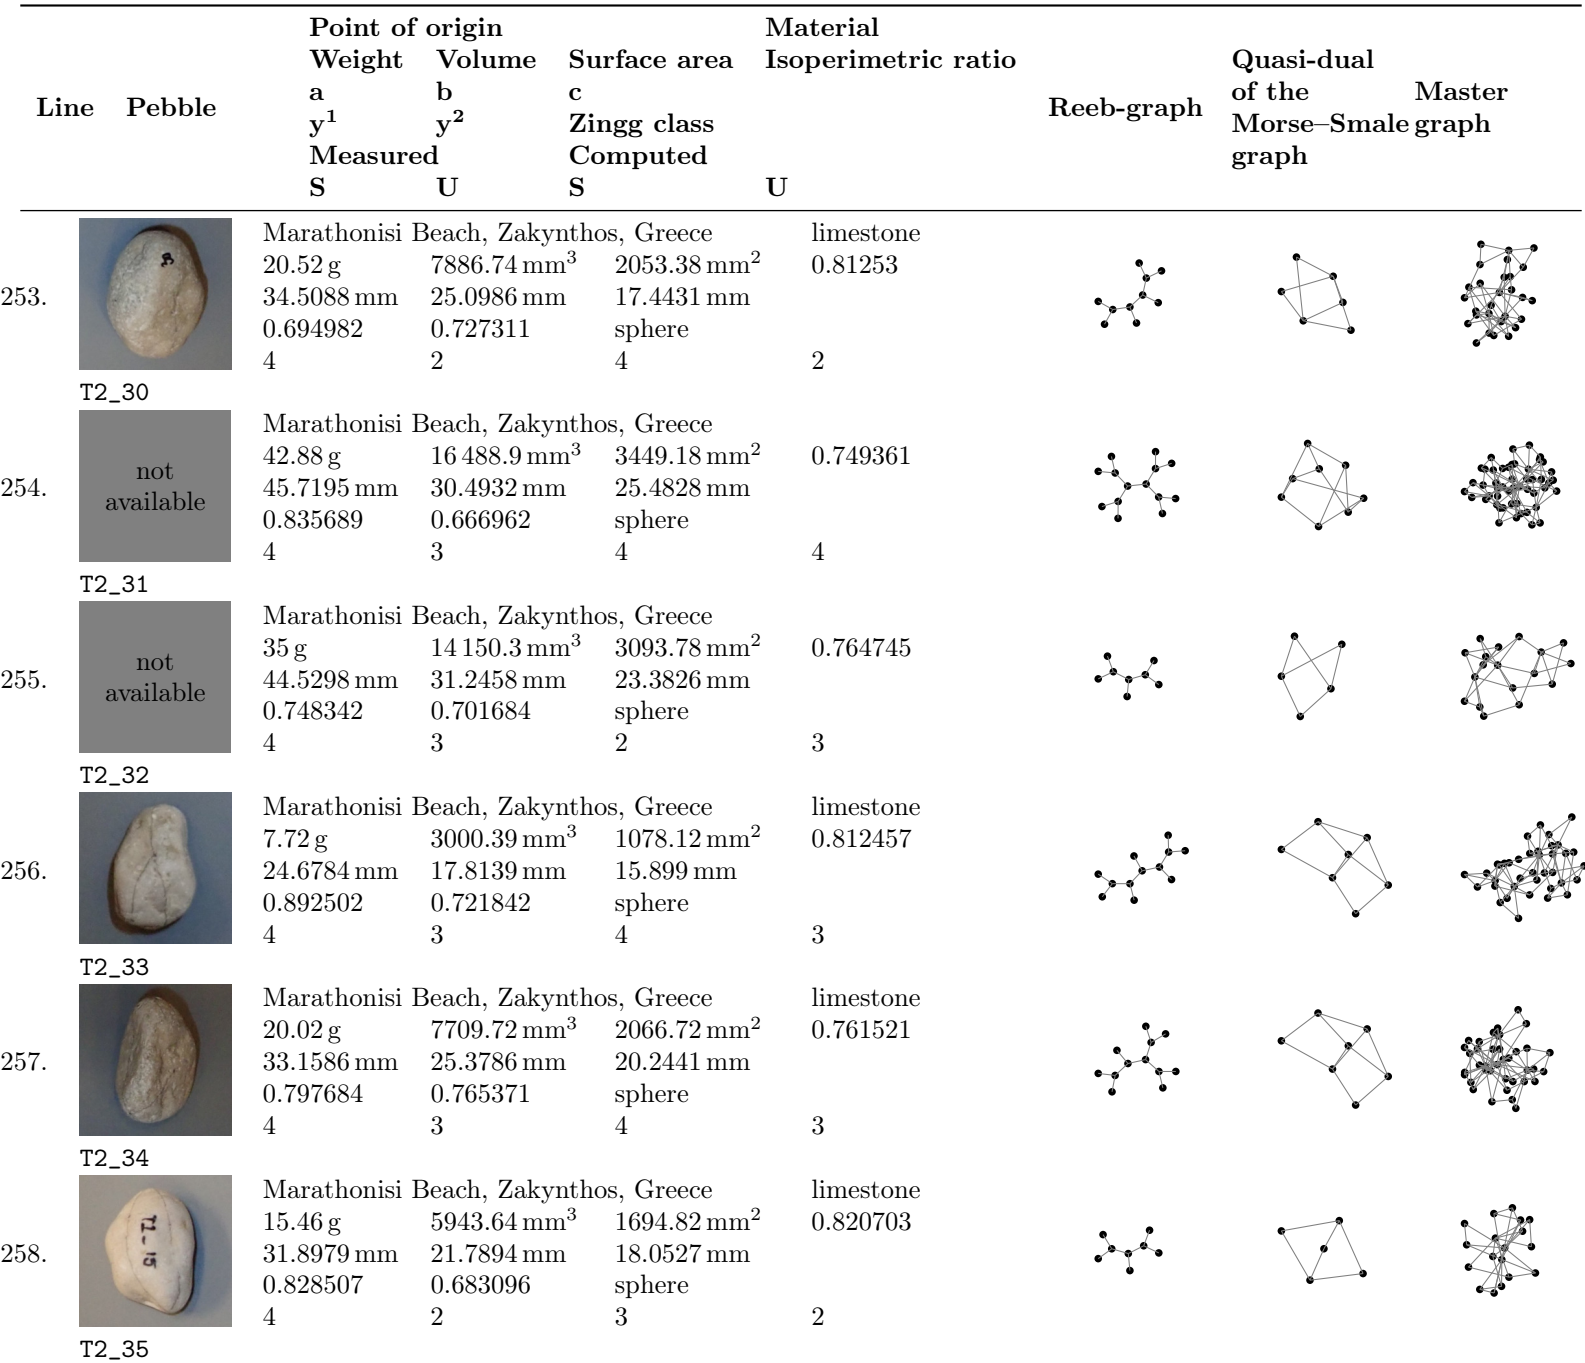 |
|      | T2_34                                                                               |                                                                                |                                                                    |                                                      |                                      |                                                                                       |                                                                                       |                                                                                       |
| 258. | 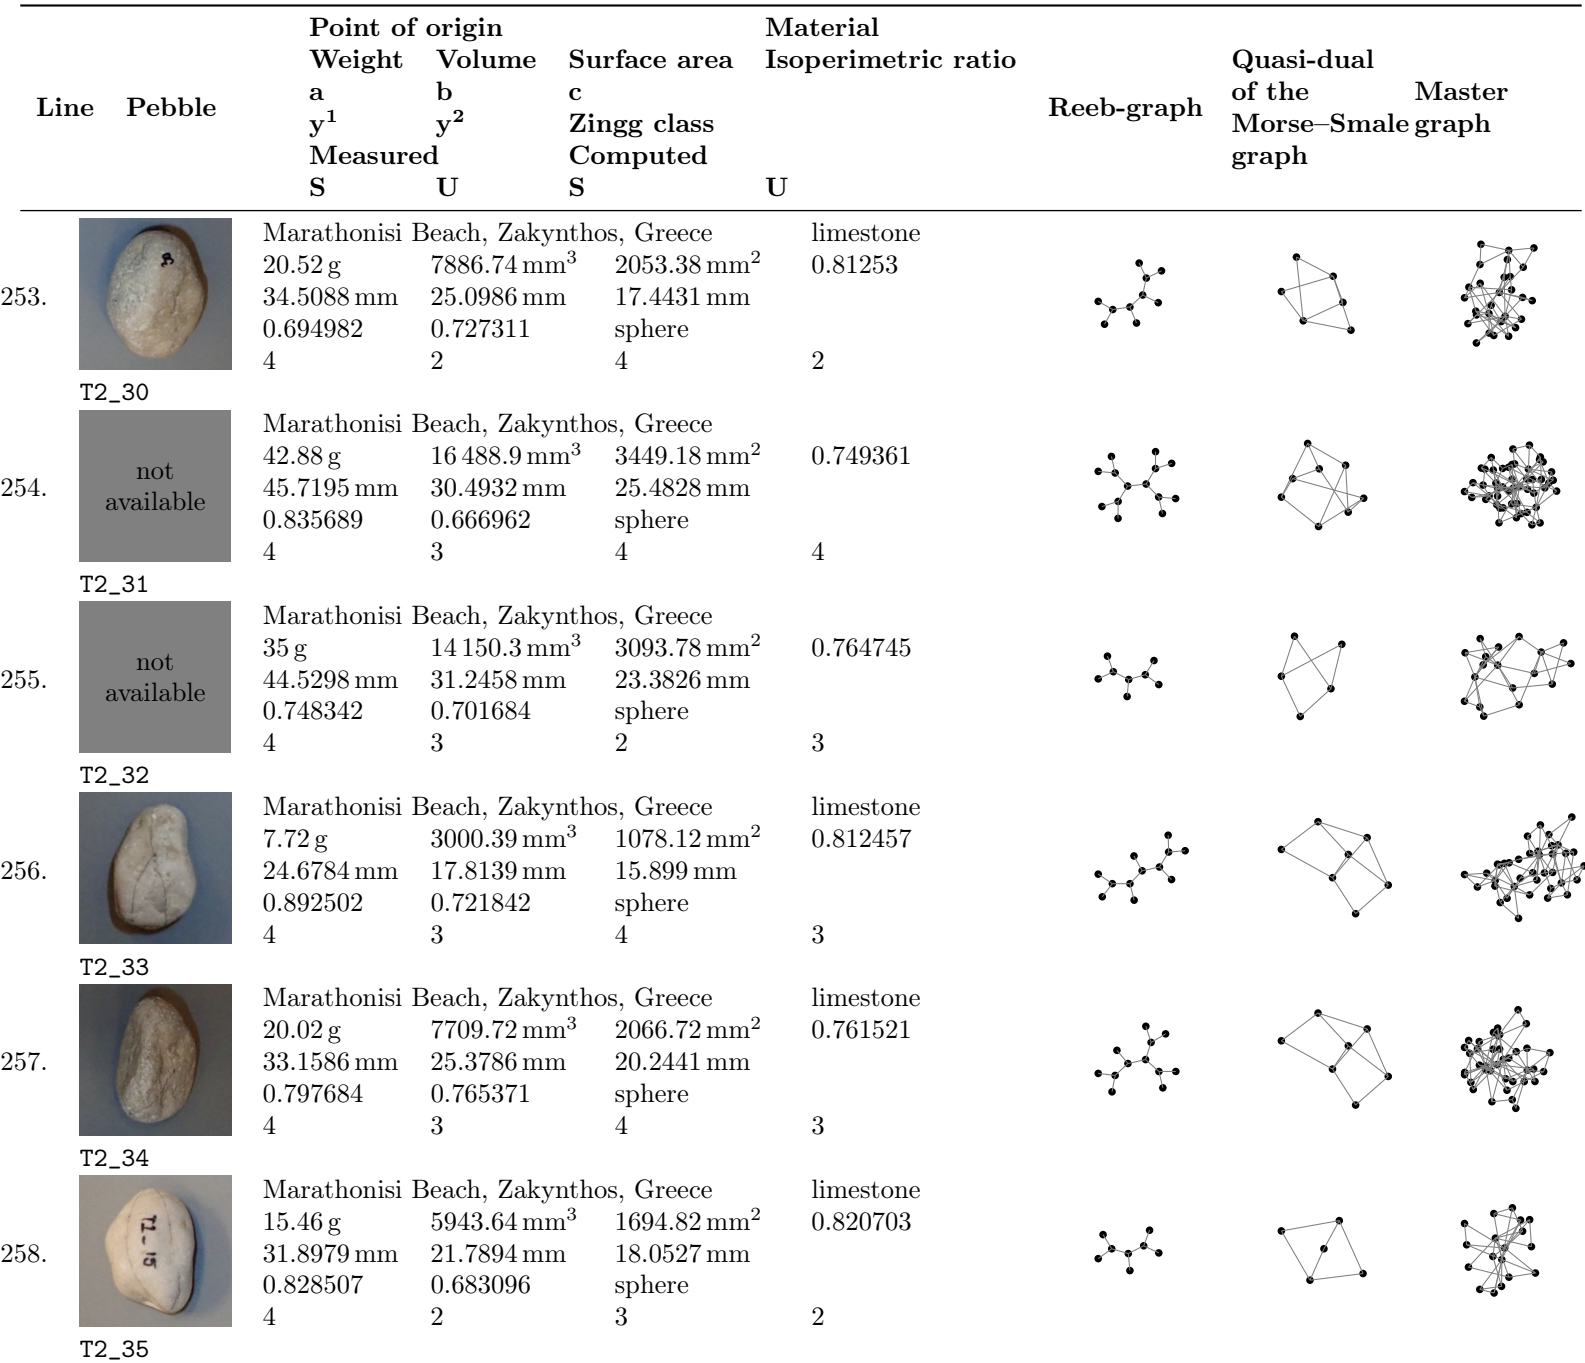 | Marathonisi Beach, Zakynthos, Greece<br>15.46 g<br>31.8979 mm<br>0.828507<br>4 | 15.46 g<br>5943.64 mm <sup>3</sup><br>21.7894 mm<br>0.683096<br>2  | 1694.82 mm <sup>2</sup><br>18.0527 mm<br>sphere<br>3 | limestone<br>0.820703<br><br>2       | 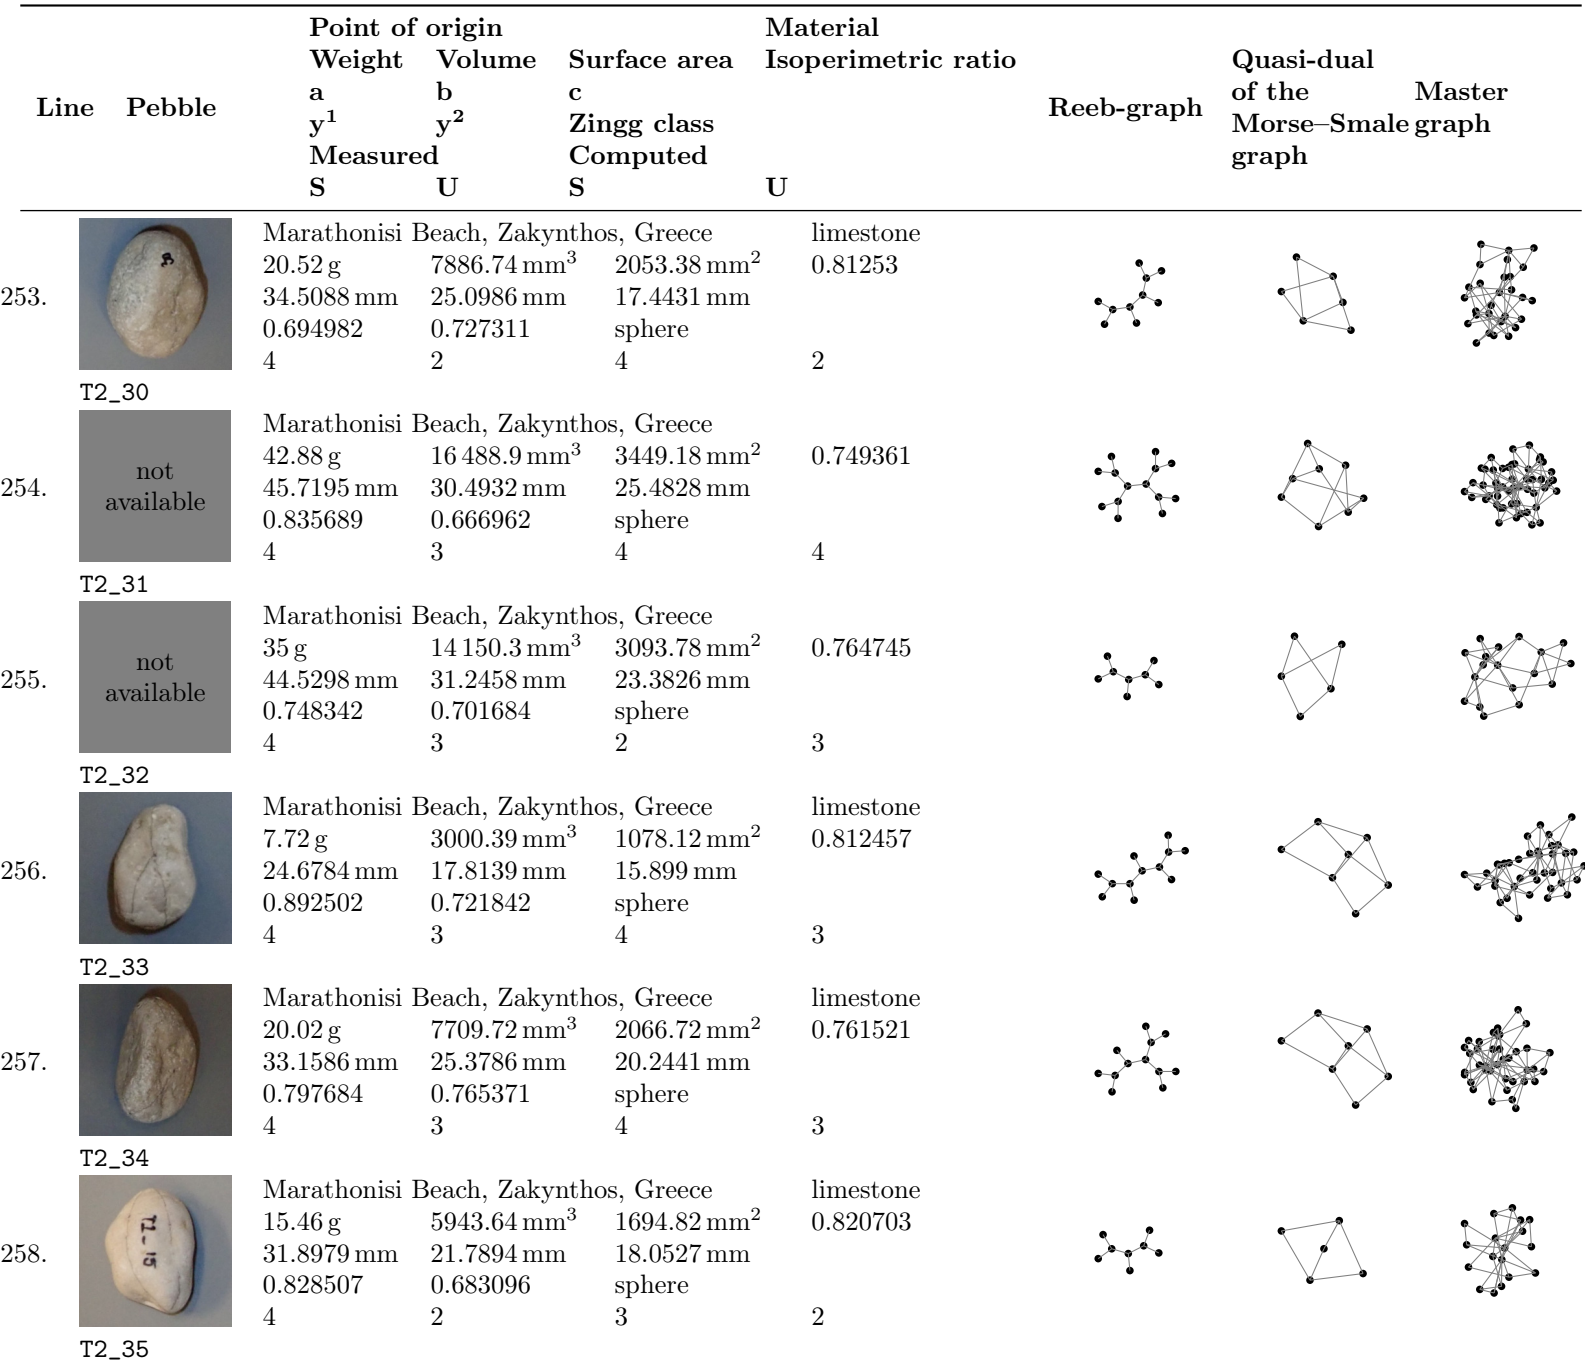 | 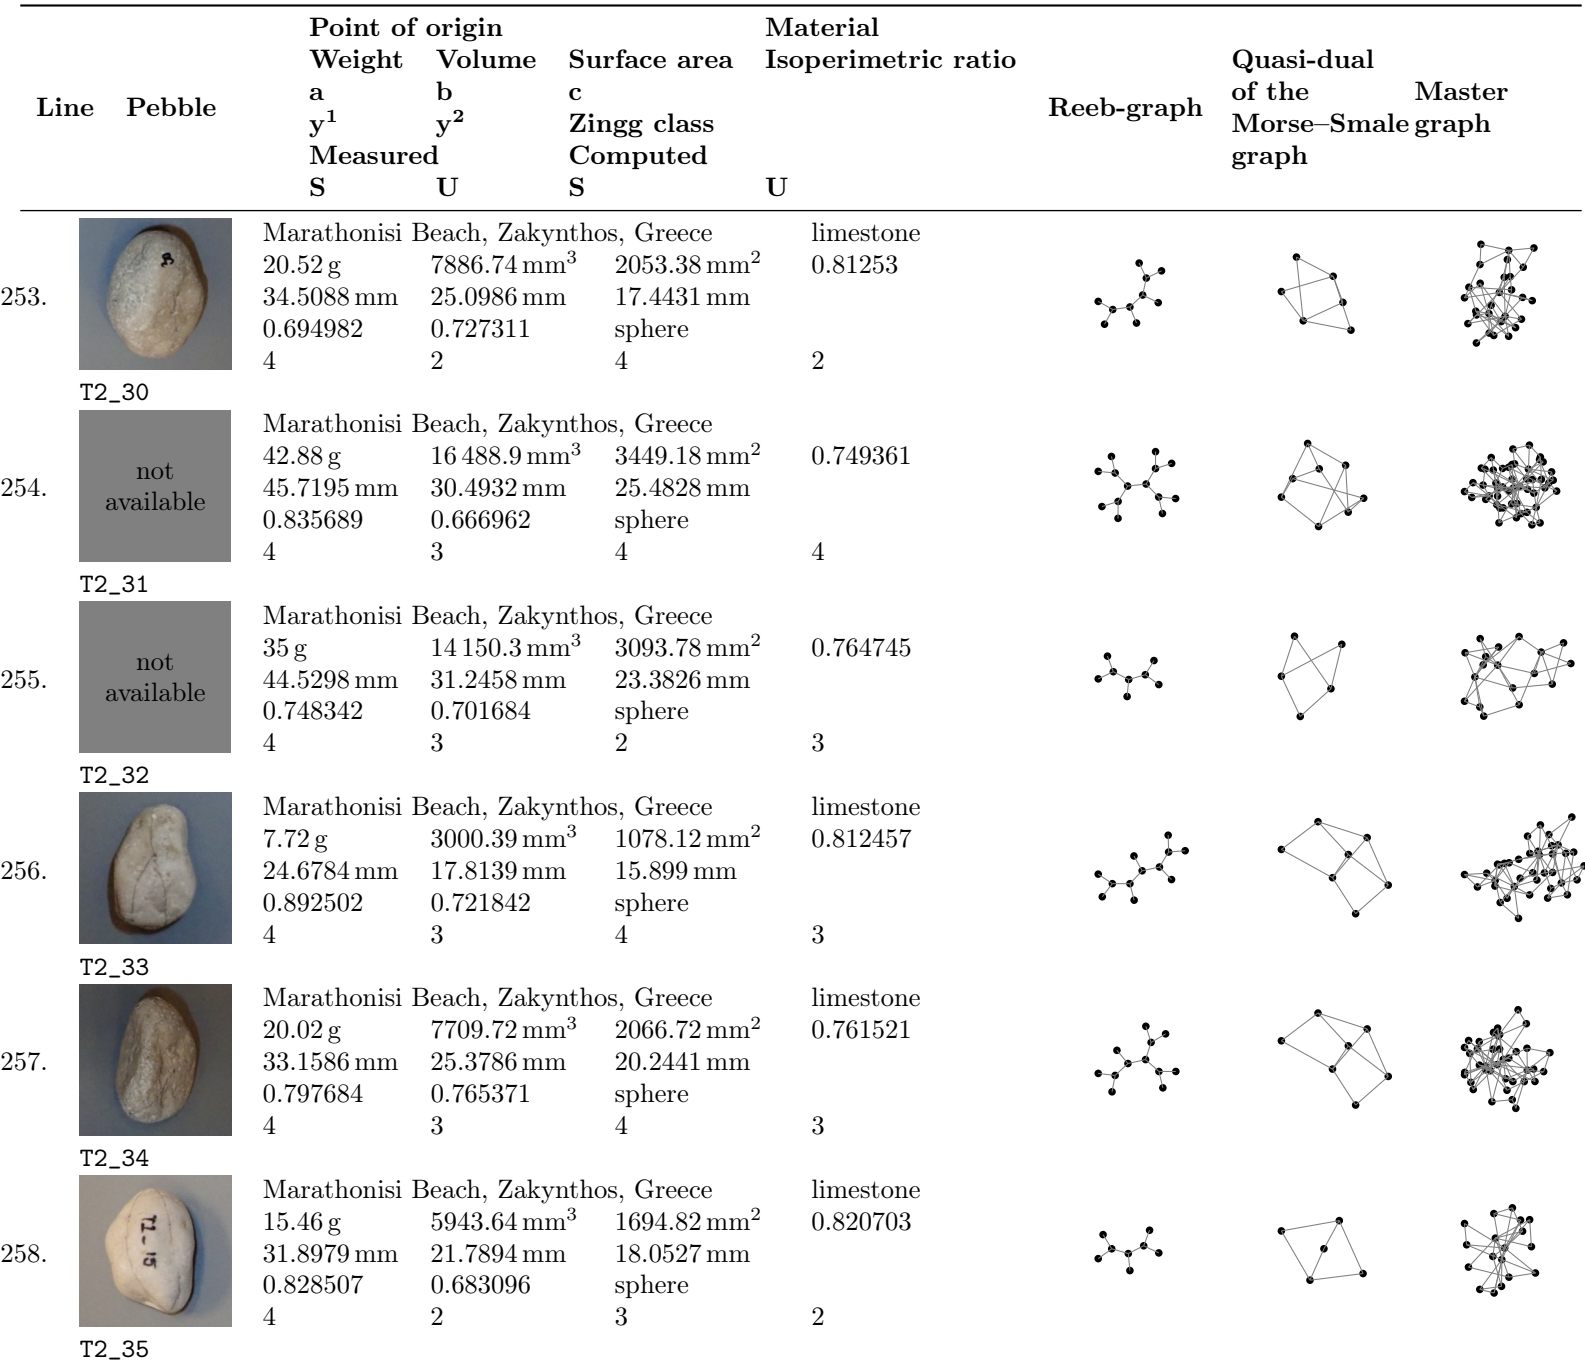 | 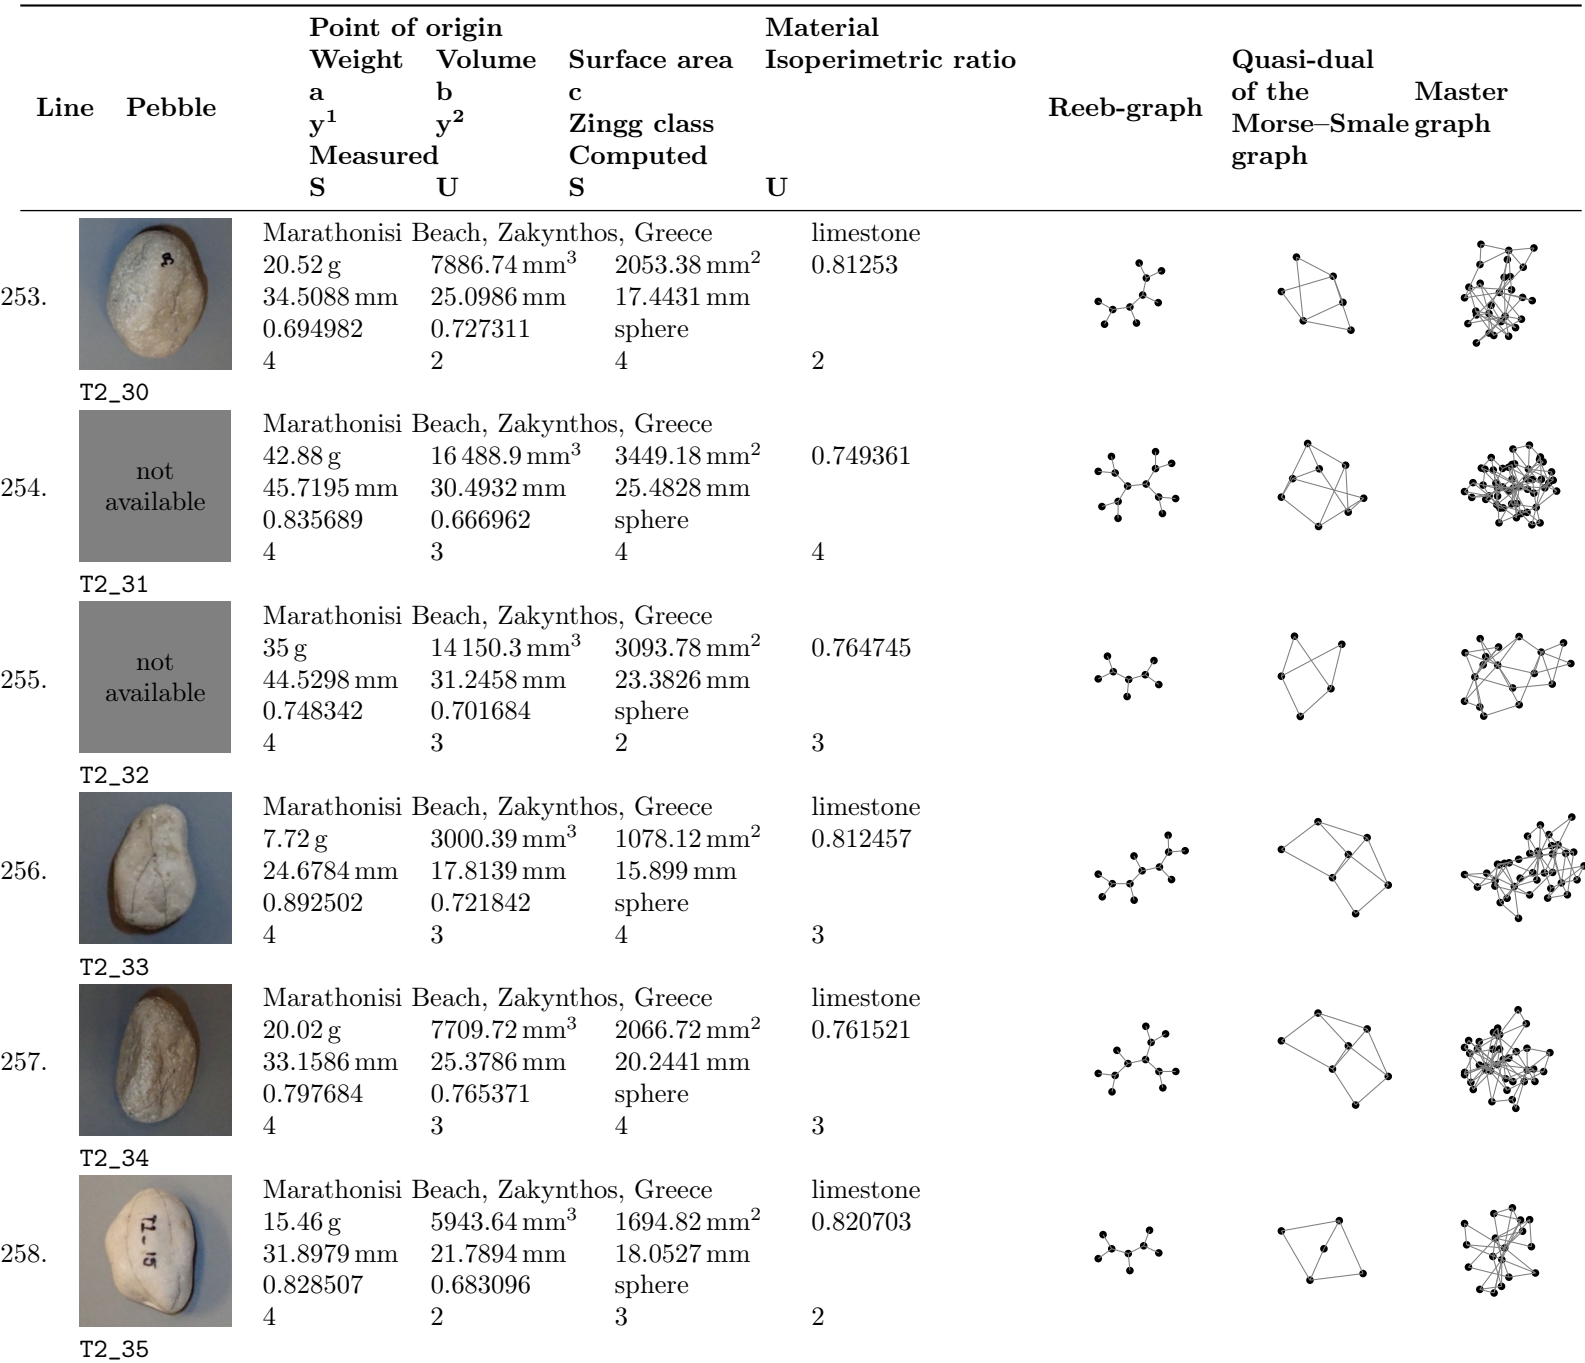 |
|      | T2_35                                                                               |                                                                                |                                                                    |                                                      |                                      |                                                                                       |                                                                                       |                                                                                       |

| Line | Pebble                                                                              | Point of origin                                                                |                                                        |                                                      | Material                       | Isoperimetric ratio | Reeb-graph                                                                            | Quasi-dual<br>of the<br>Morse–Smale<br>graph                                          | Master                                                                                |
|------|-------------------------------------------------------------------------------------|--------------------------------------------------------------------------------|--------------------------------------------------------|------------------------------------------------------|--------------------------------|---------------------|---------------------------------------------------------------------------------------|---------------------------------------------------------------------------------------|---------------------------------------------------------------------------------------|
|      |                                                                                     | Weight                                                                         | Volume                                                 | Surface area                                         |                                |                     |                                                                                       |                                                                                       |                                                                                       |
|      |                                                                                     | a                                                                              | b                                                      | c                                                    |                                |                     |                                                                                       |                                                                                       |                                                                                       |
|      |                                                                                     | y <sup>1</sup><br>Measured<br>S                                                | y <sup>2</sup><br>U                                    | Zingg class<br>Computed<br>S                         |                                |                     |                                                                                       |                                                                                       |                                                                                       |
| 259. | 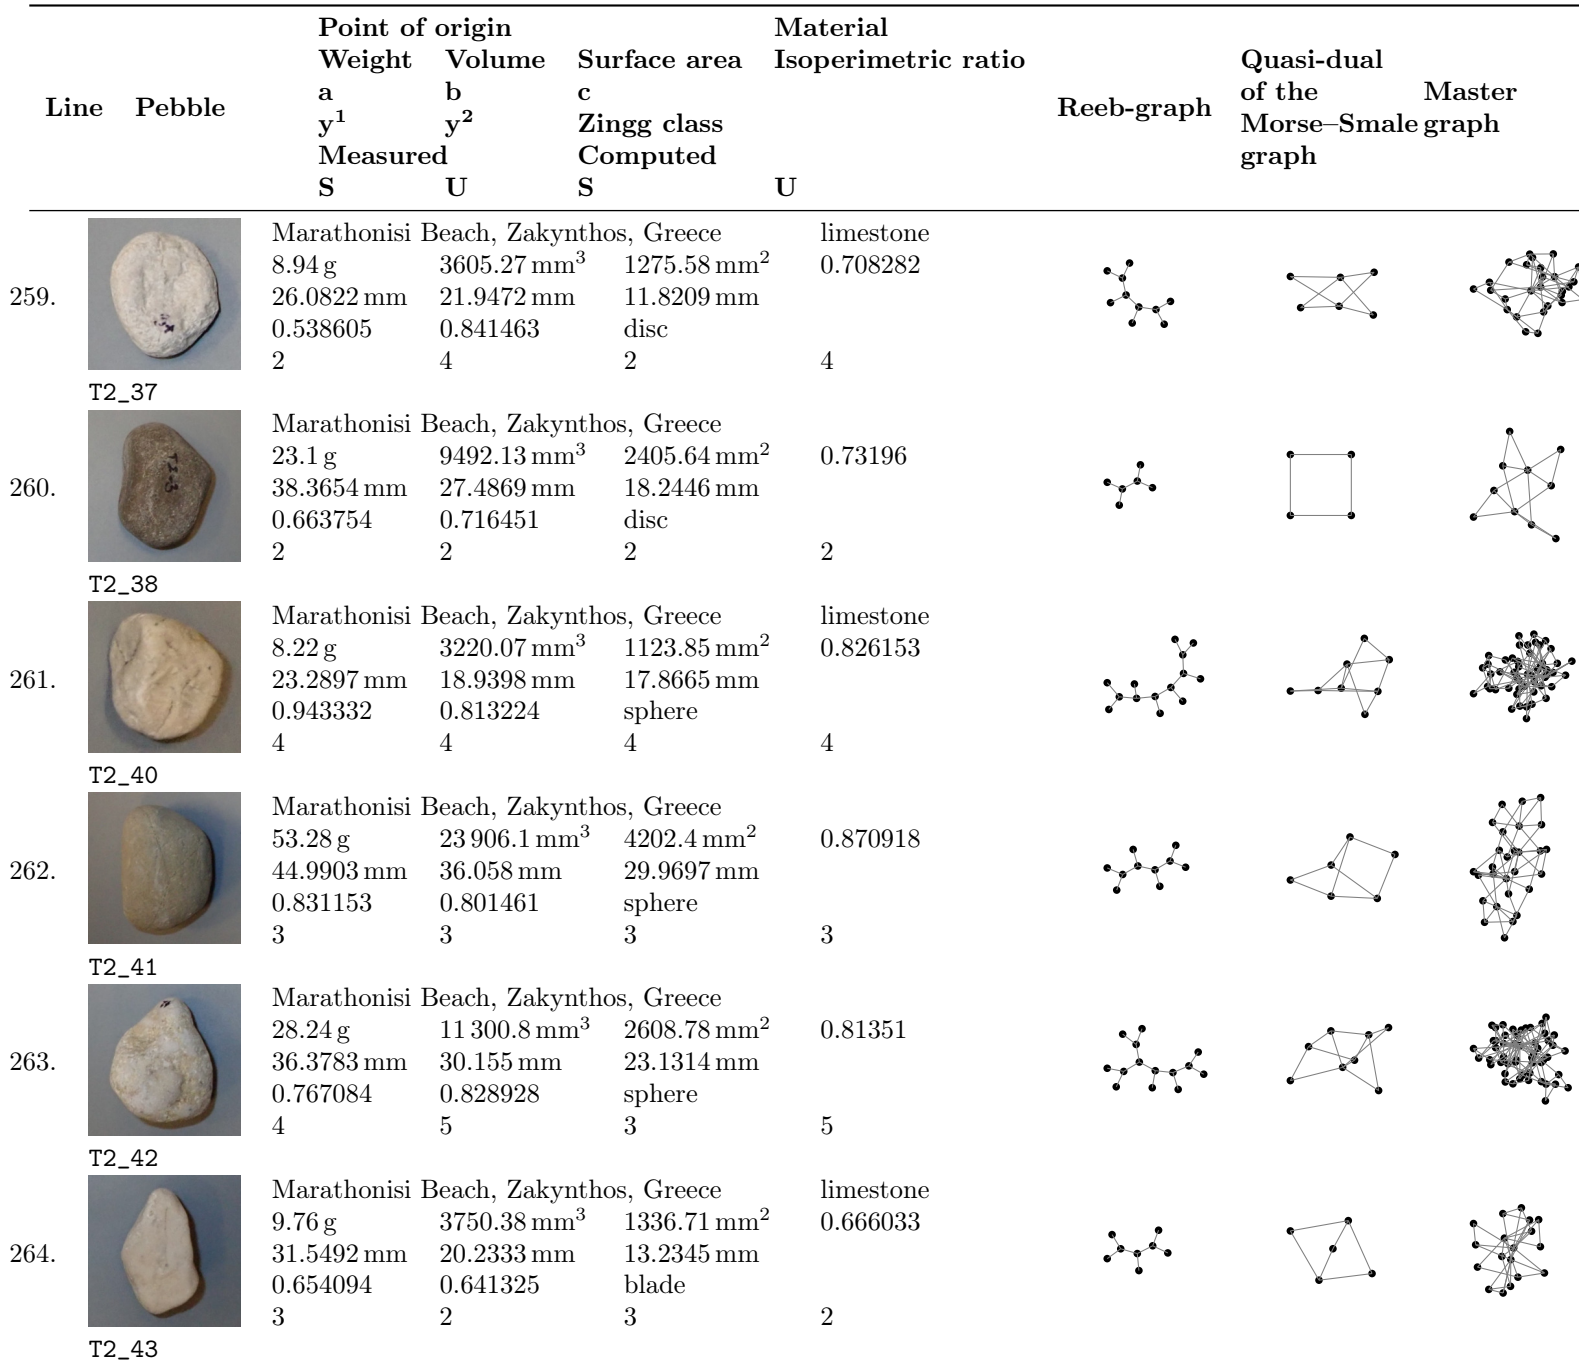   | Marathonisi Beach, Zakynthos, Greece<br>8.94 g<br>26.0822 mm<br>0.538605<br>2  | 3605.27 mm <sup>3</sup><br>21.9472 mm<br>0.841463<br>4 | 1275.58 mm <sup>2</sup><br>11.8209 mm<br>disc<br>2   | limestone<br>0.708282<br><br>4 |                     | 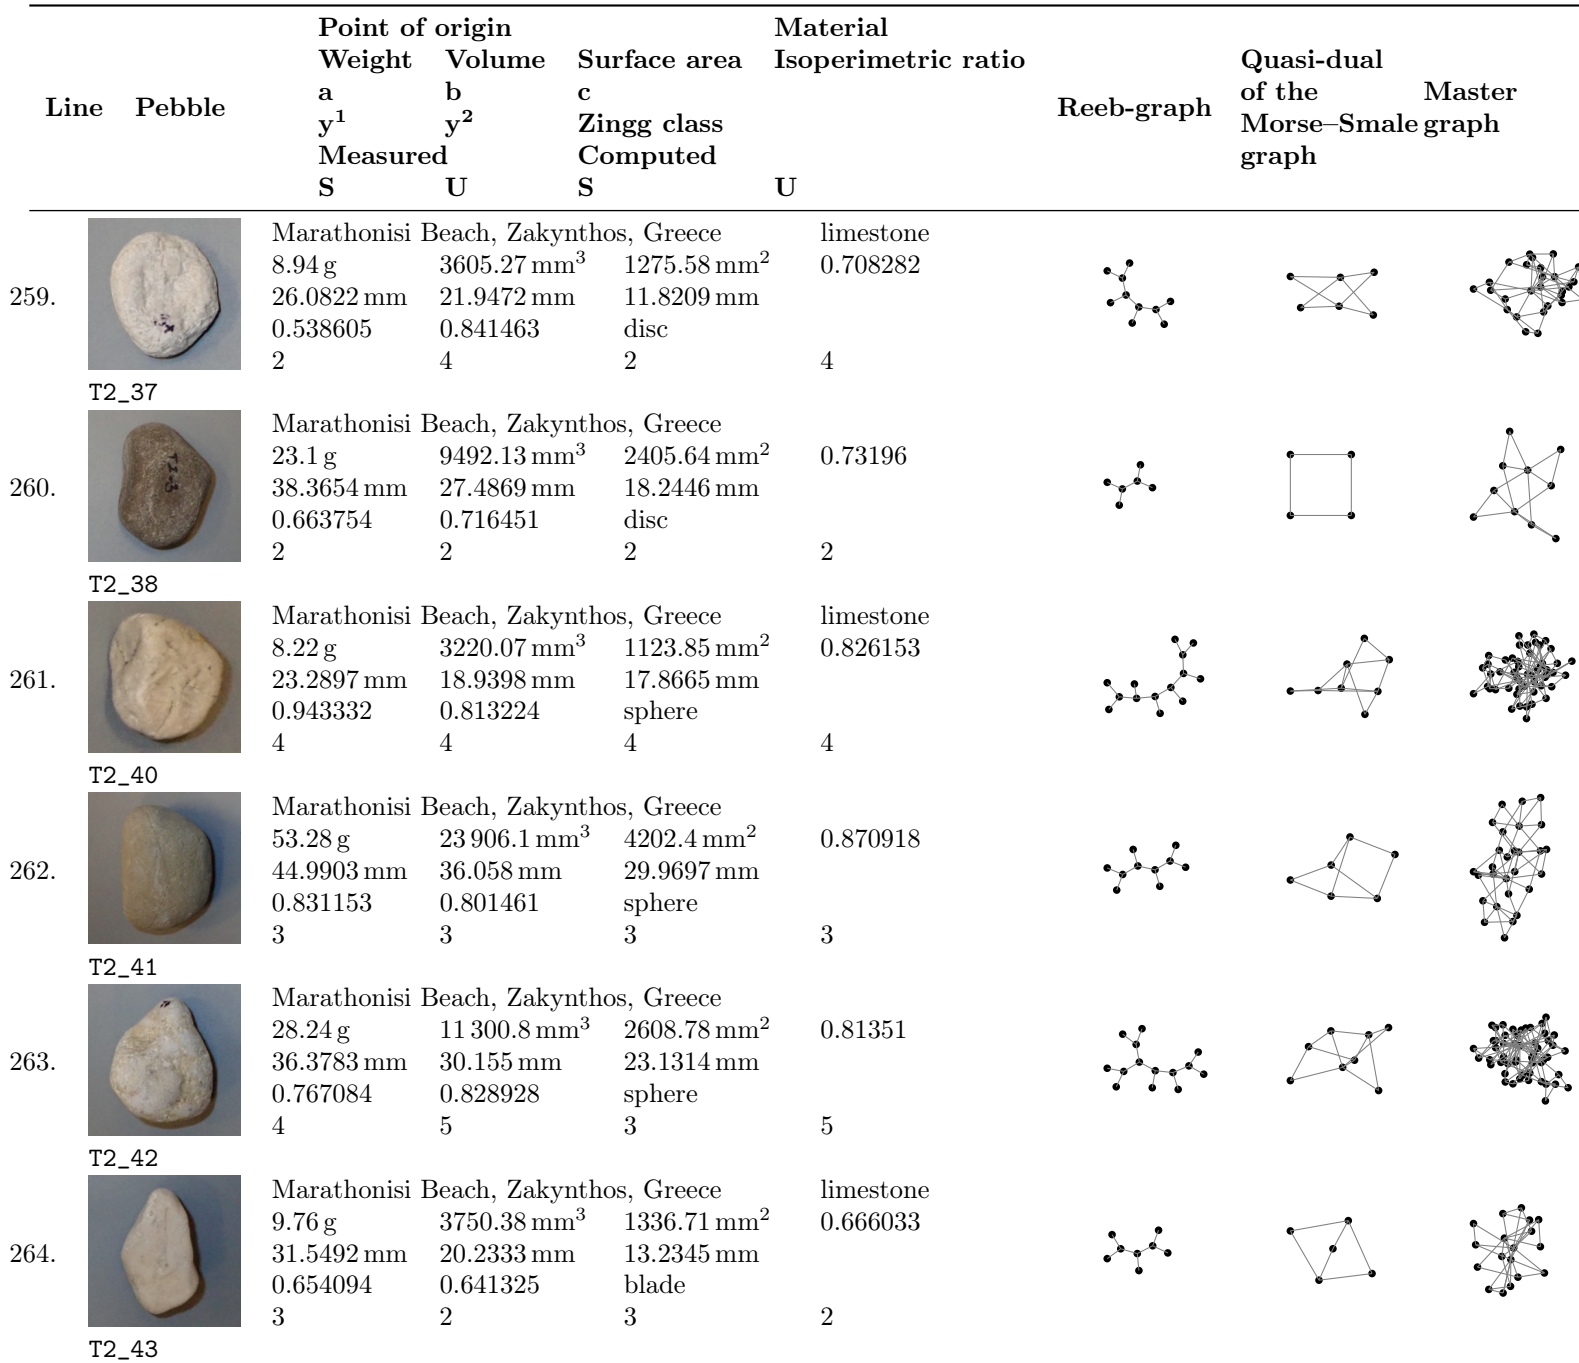   | 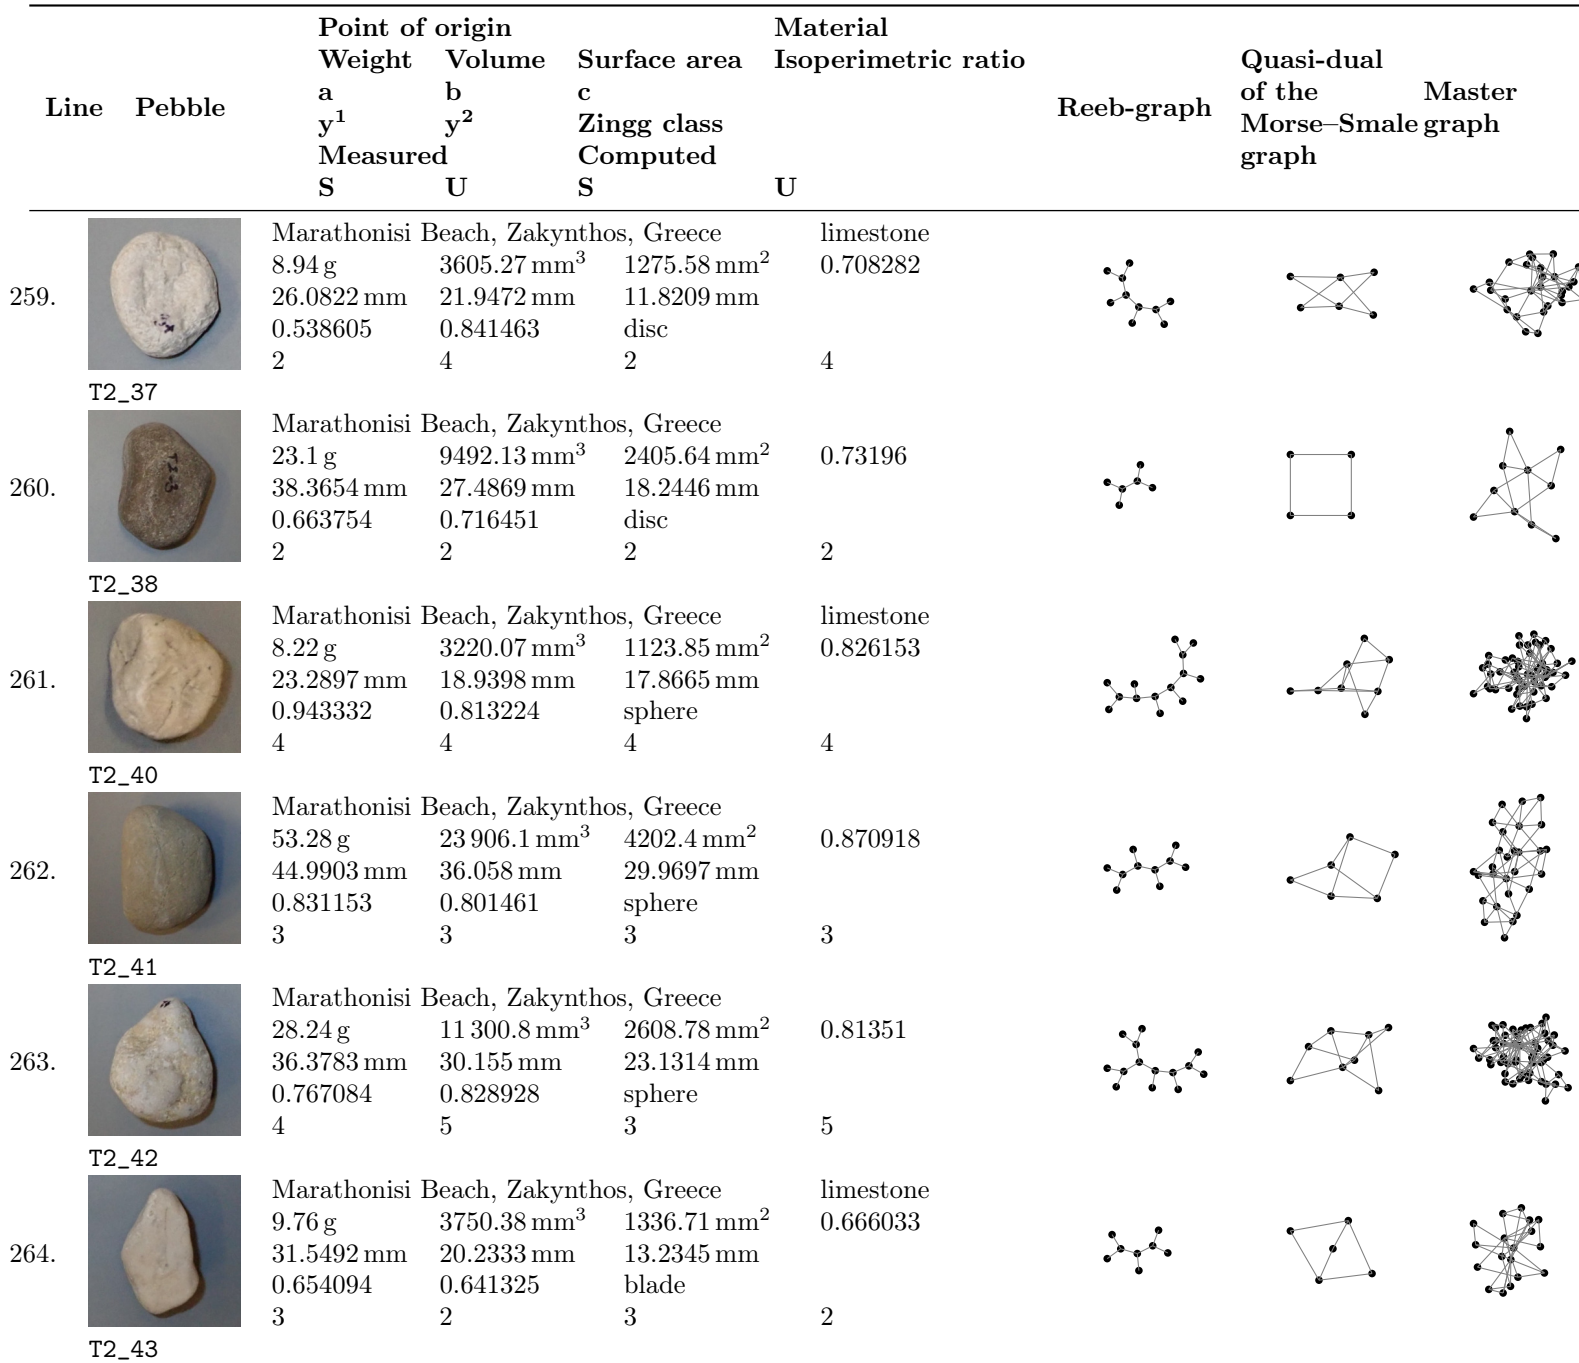   | 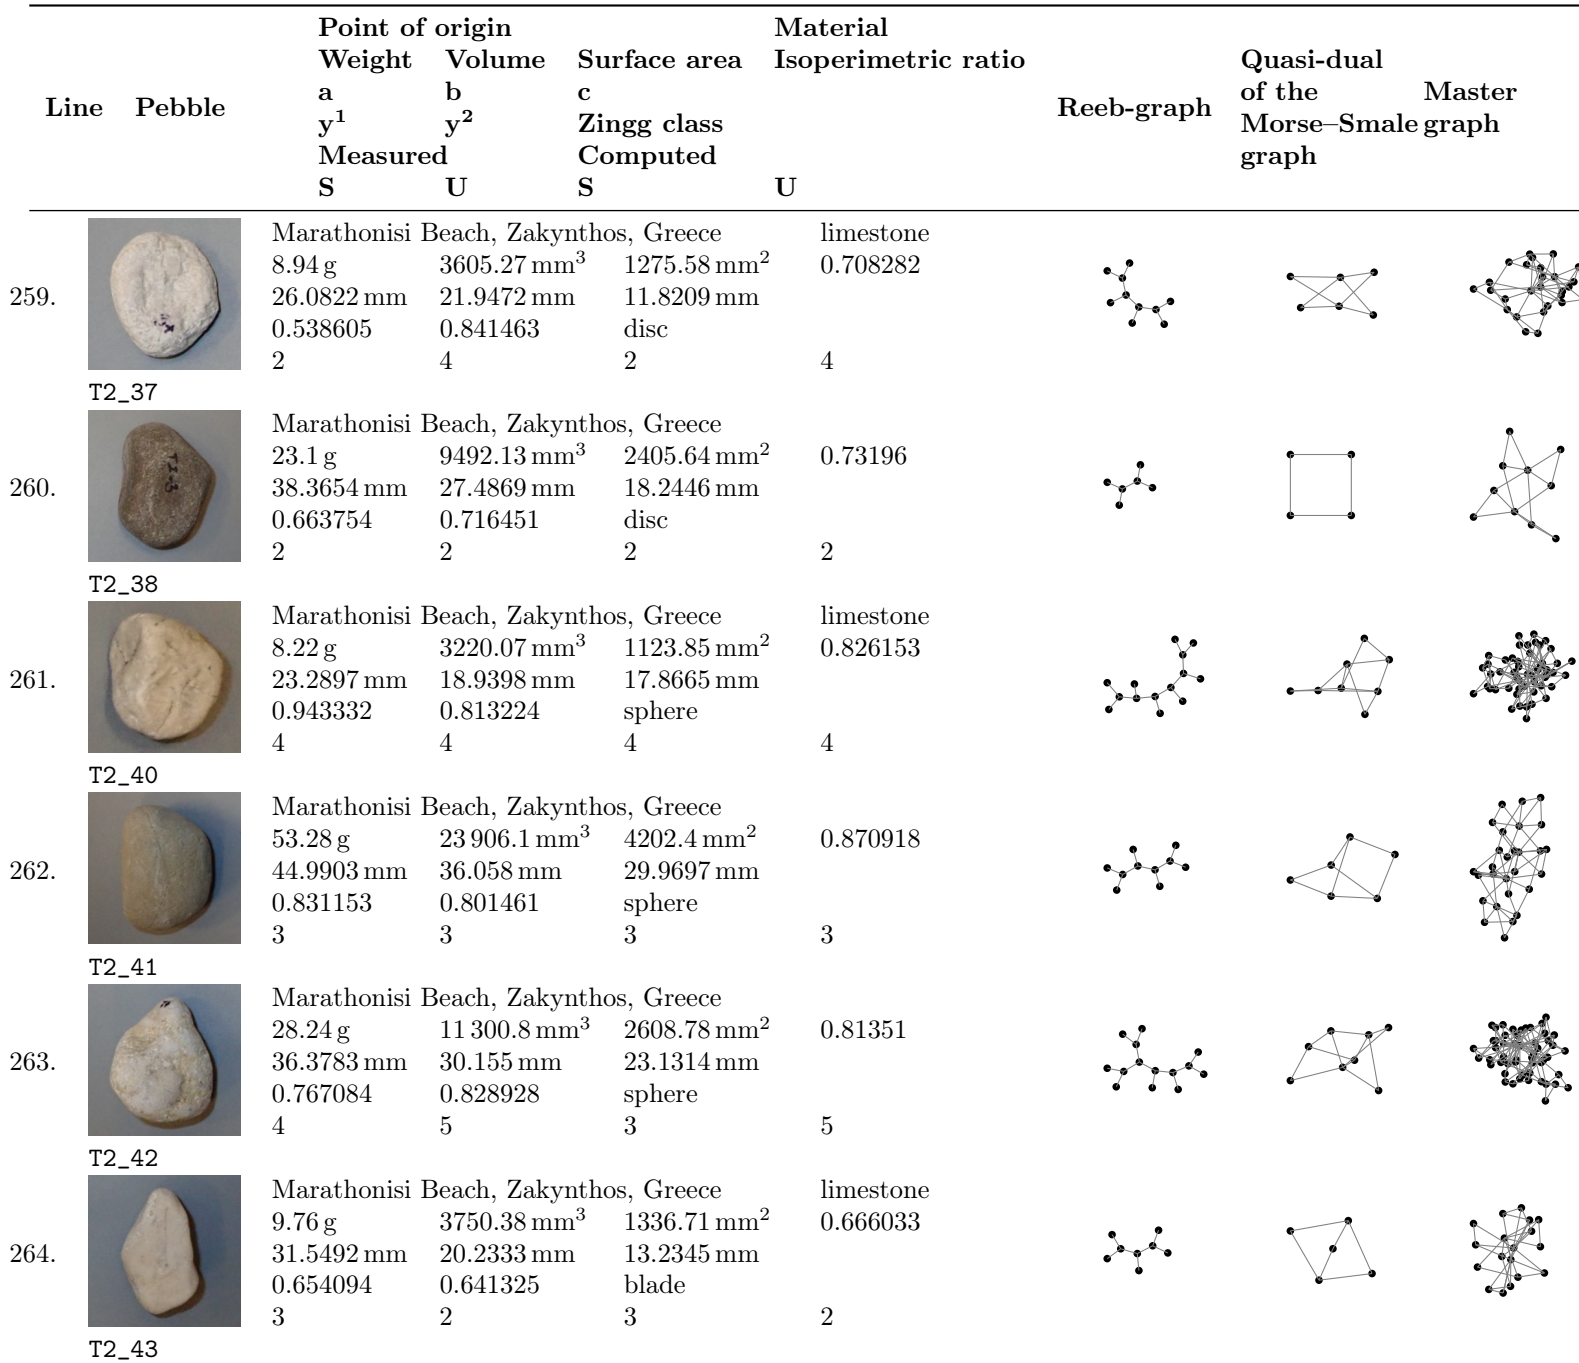   |
|      | T2_37                                                                               |                                                                                |                                                        |                                                      |                                |                     |                                                                                       |                                                                                       |                                                                                       |
| 260. | 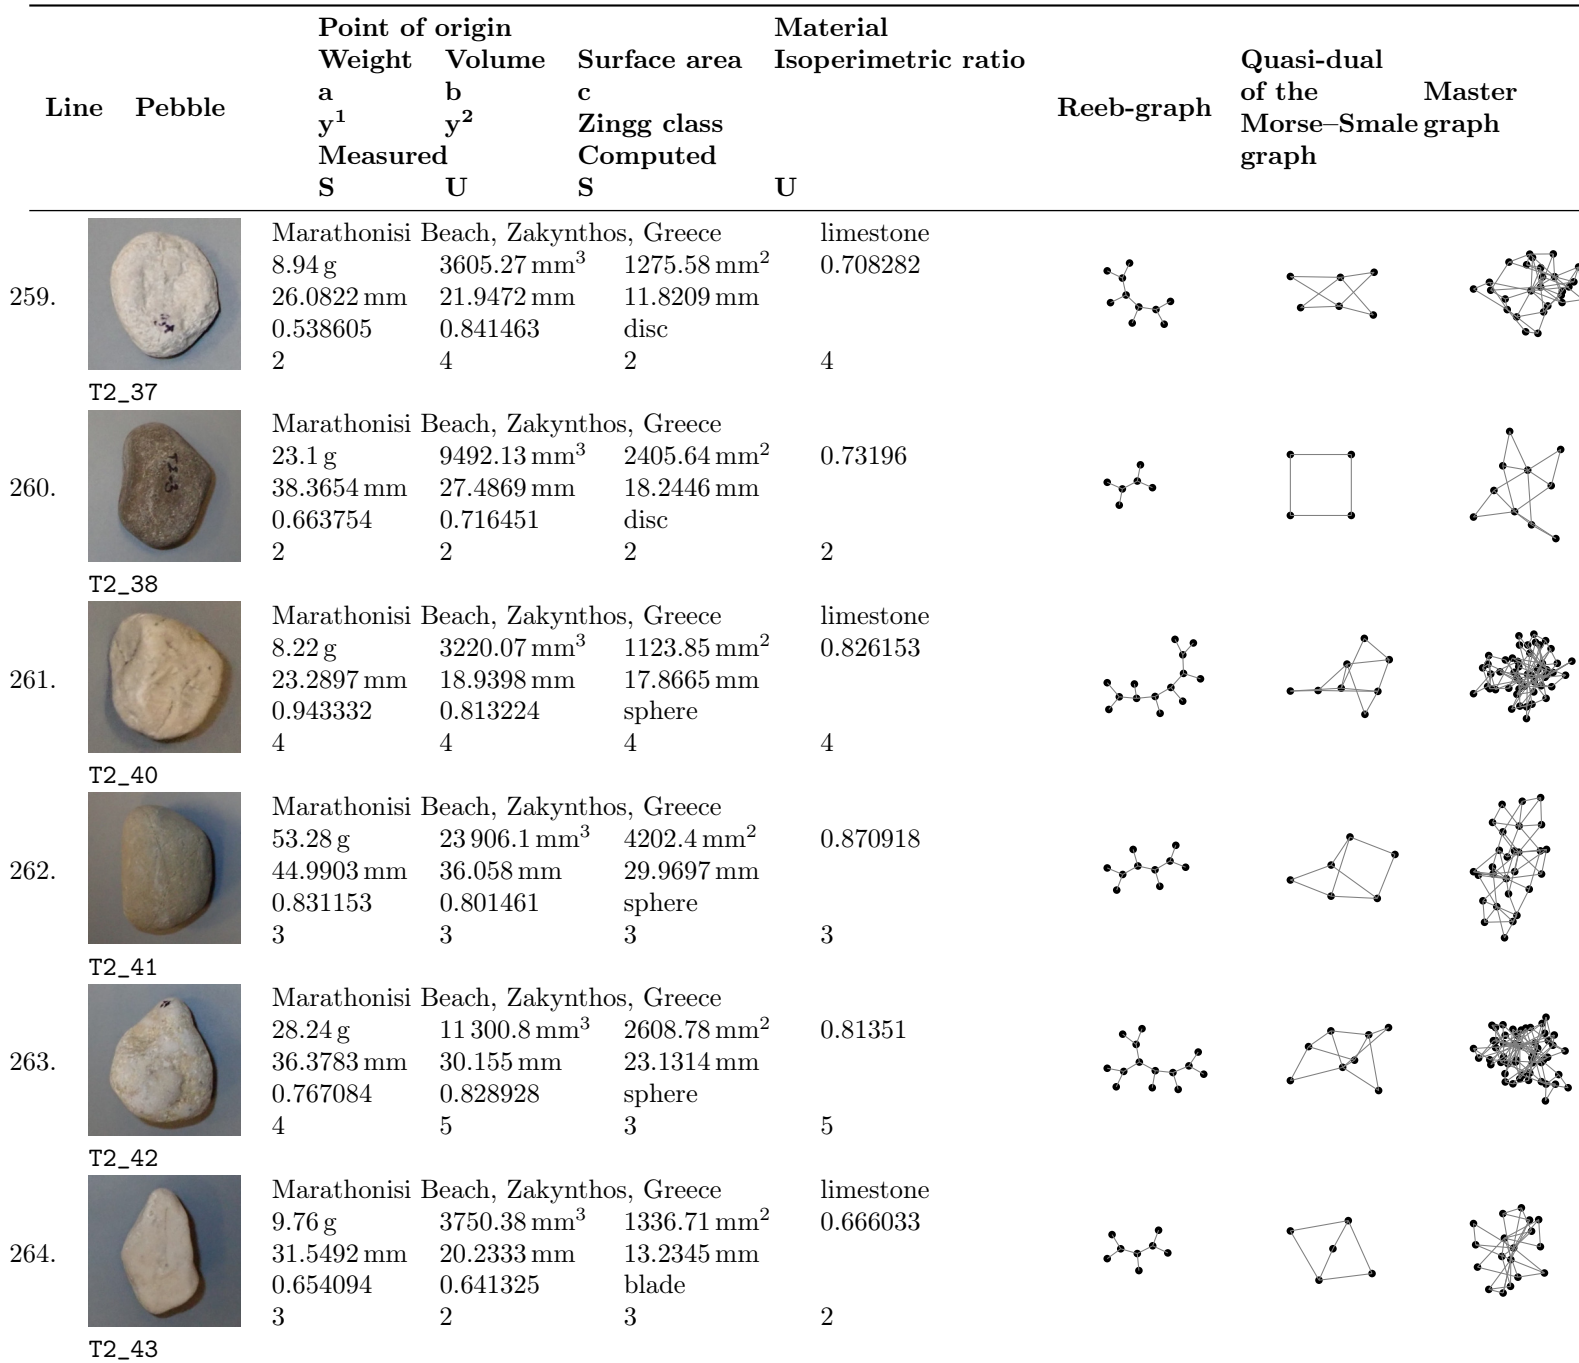   | Marathonisi Beach, Zakynthos, Greece<br>23.1 g<br>38.3654 mm<br>0.663754<br>2  | 9492.13 mm <sup>3</sup><br>27.4869 mm<br>0.716451<br>2 | 2405.64 mm <sup>2</sup><br>18.2446 mm<br>disc<br>2   | 0.73196<br><br>2               |                     | 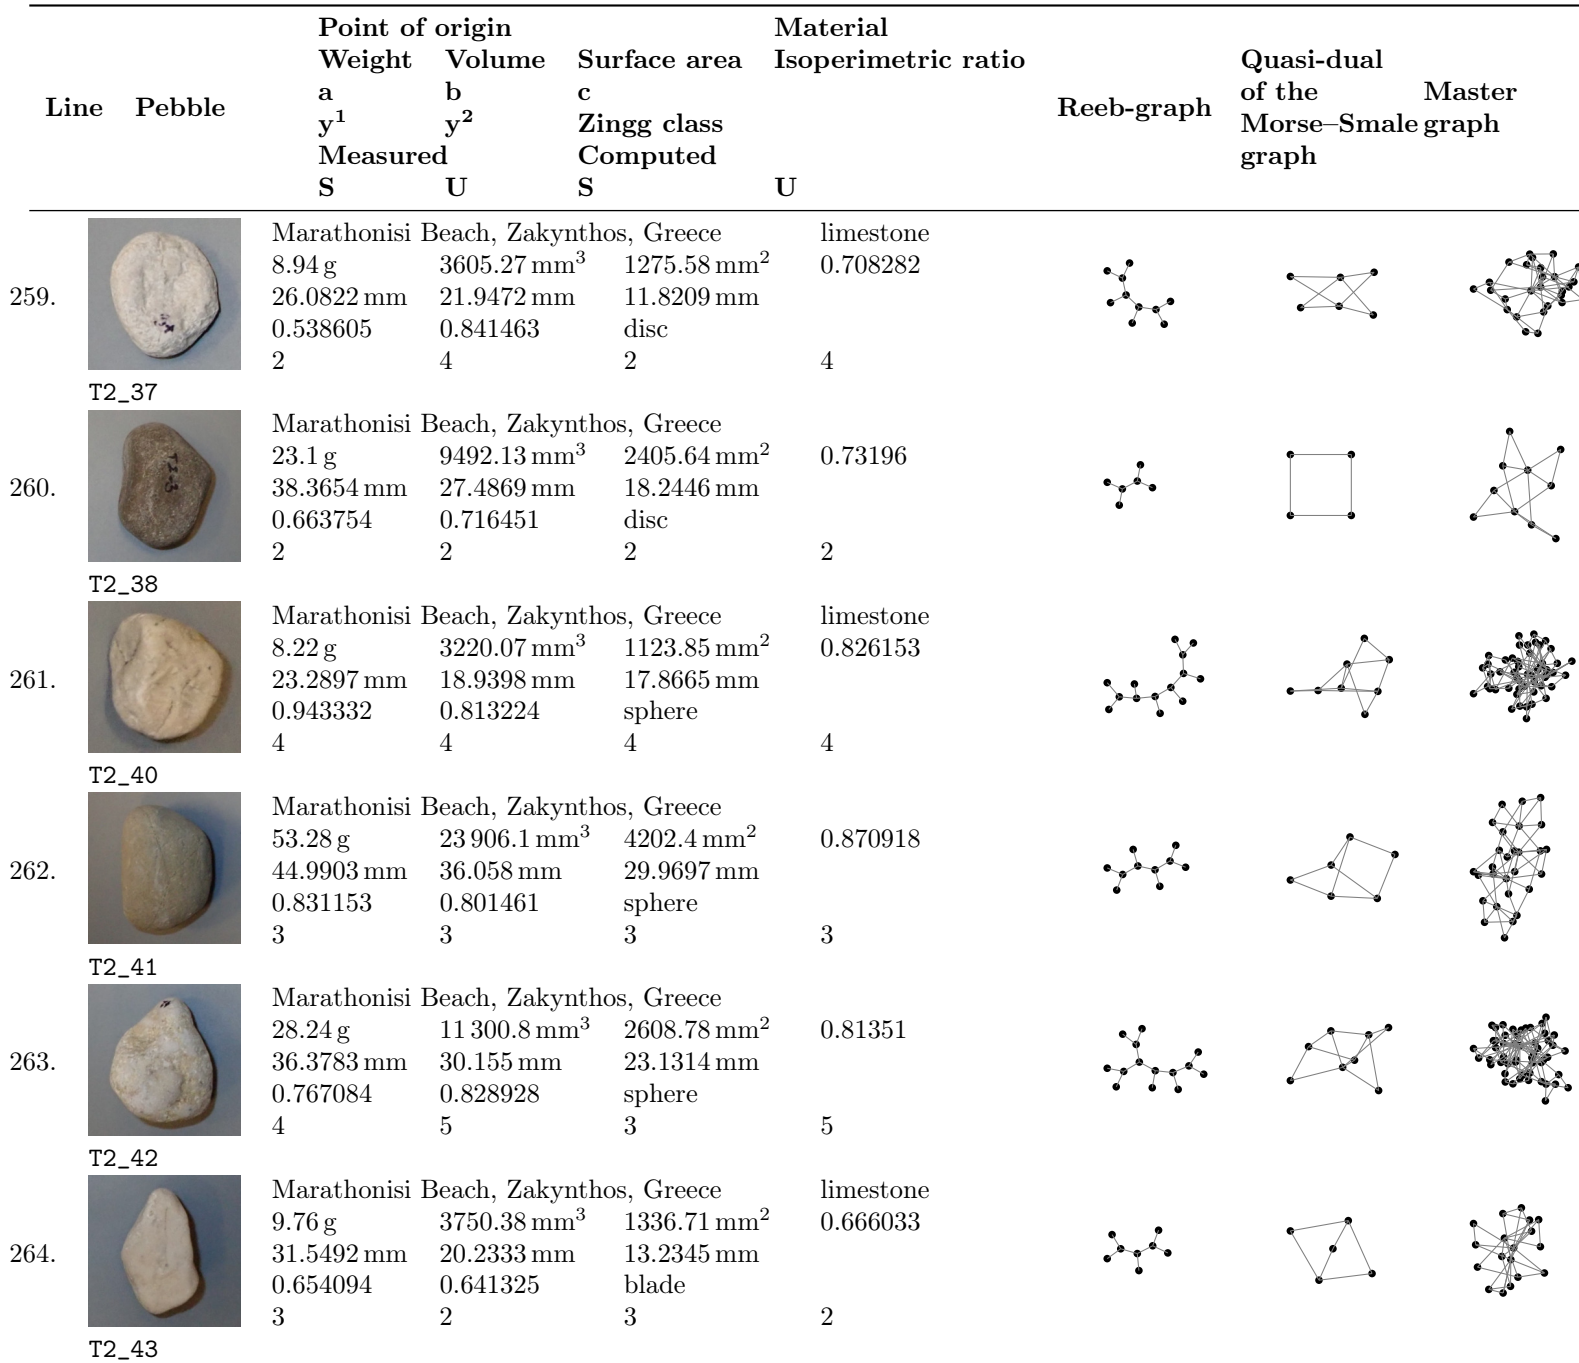   | 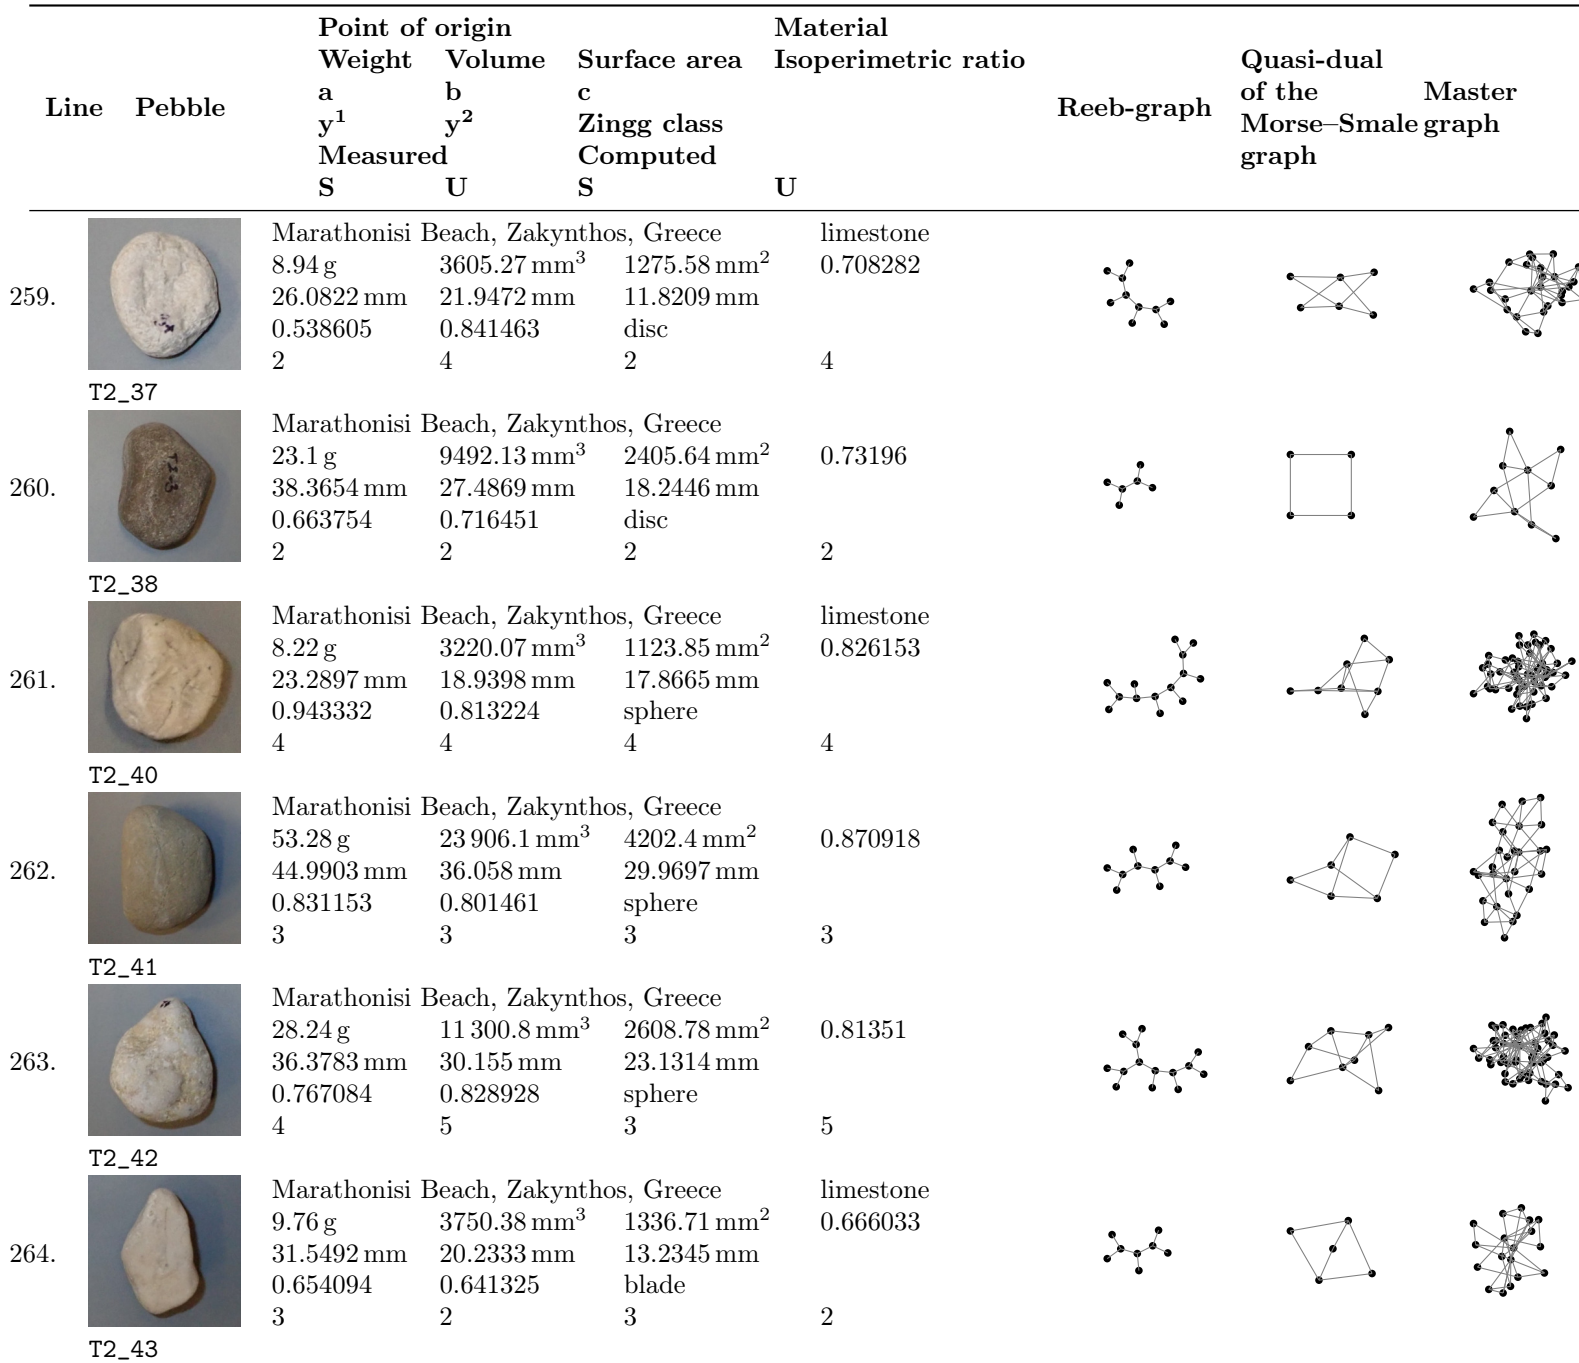   | 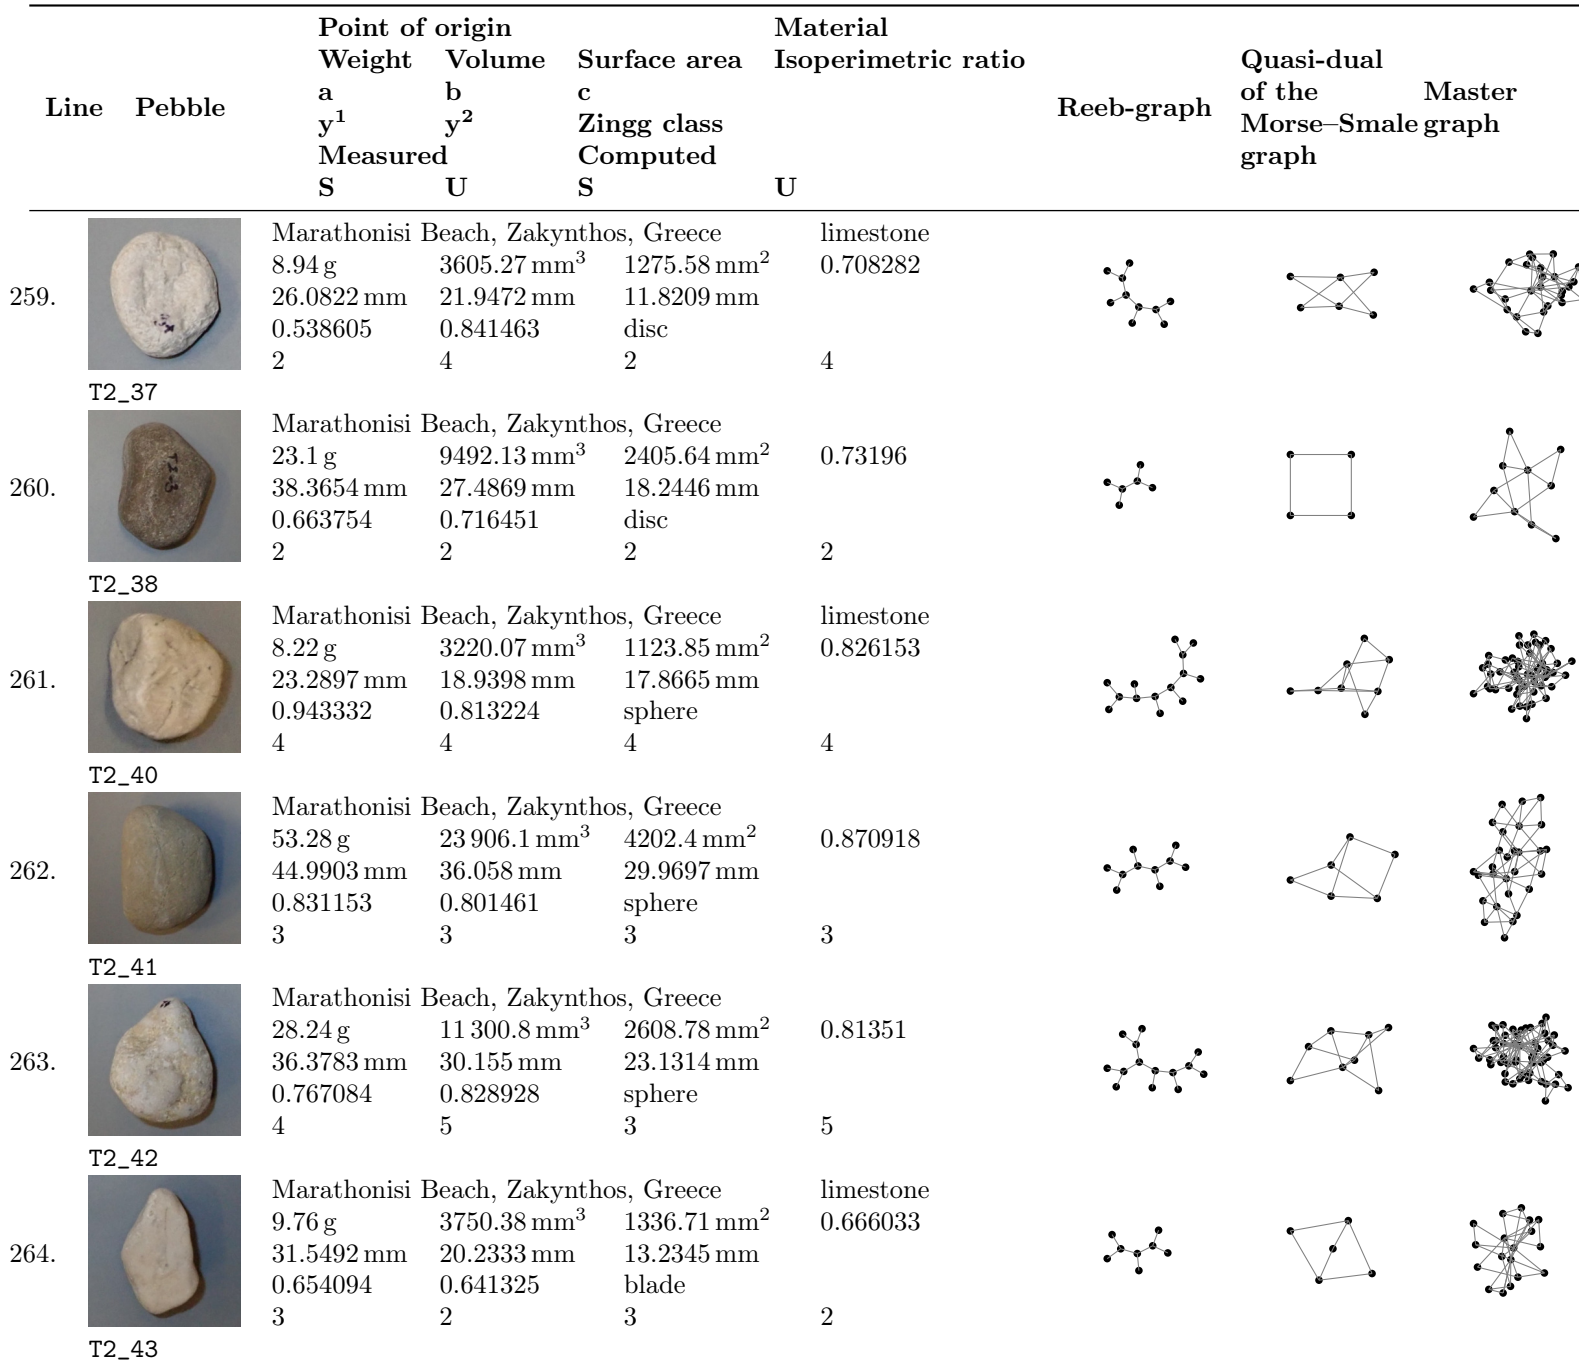   |
|      | T2_38                                                                               |                                                                                |                                                        |                                                      |                                |                     |                                                                                       |                                                                                       |                                                                                       |
| 261. | 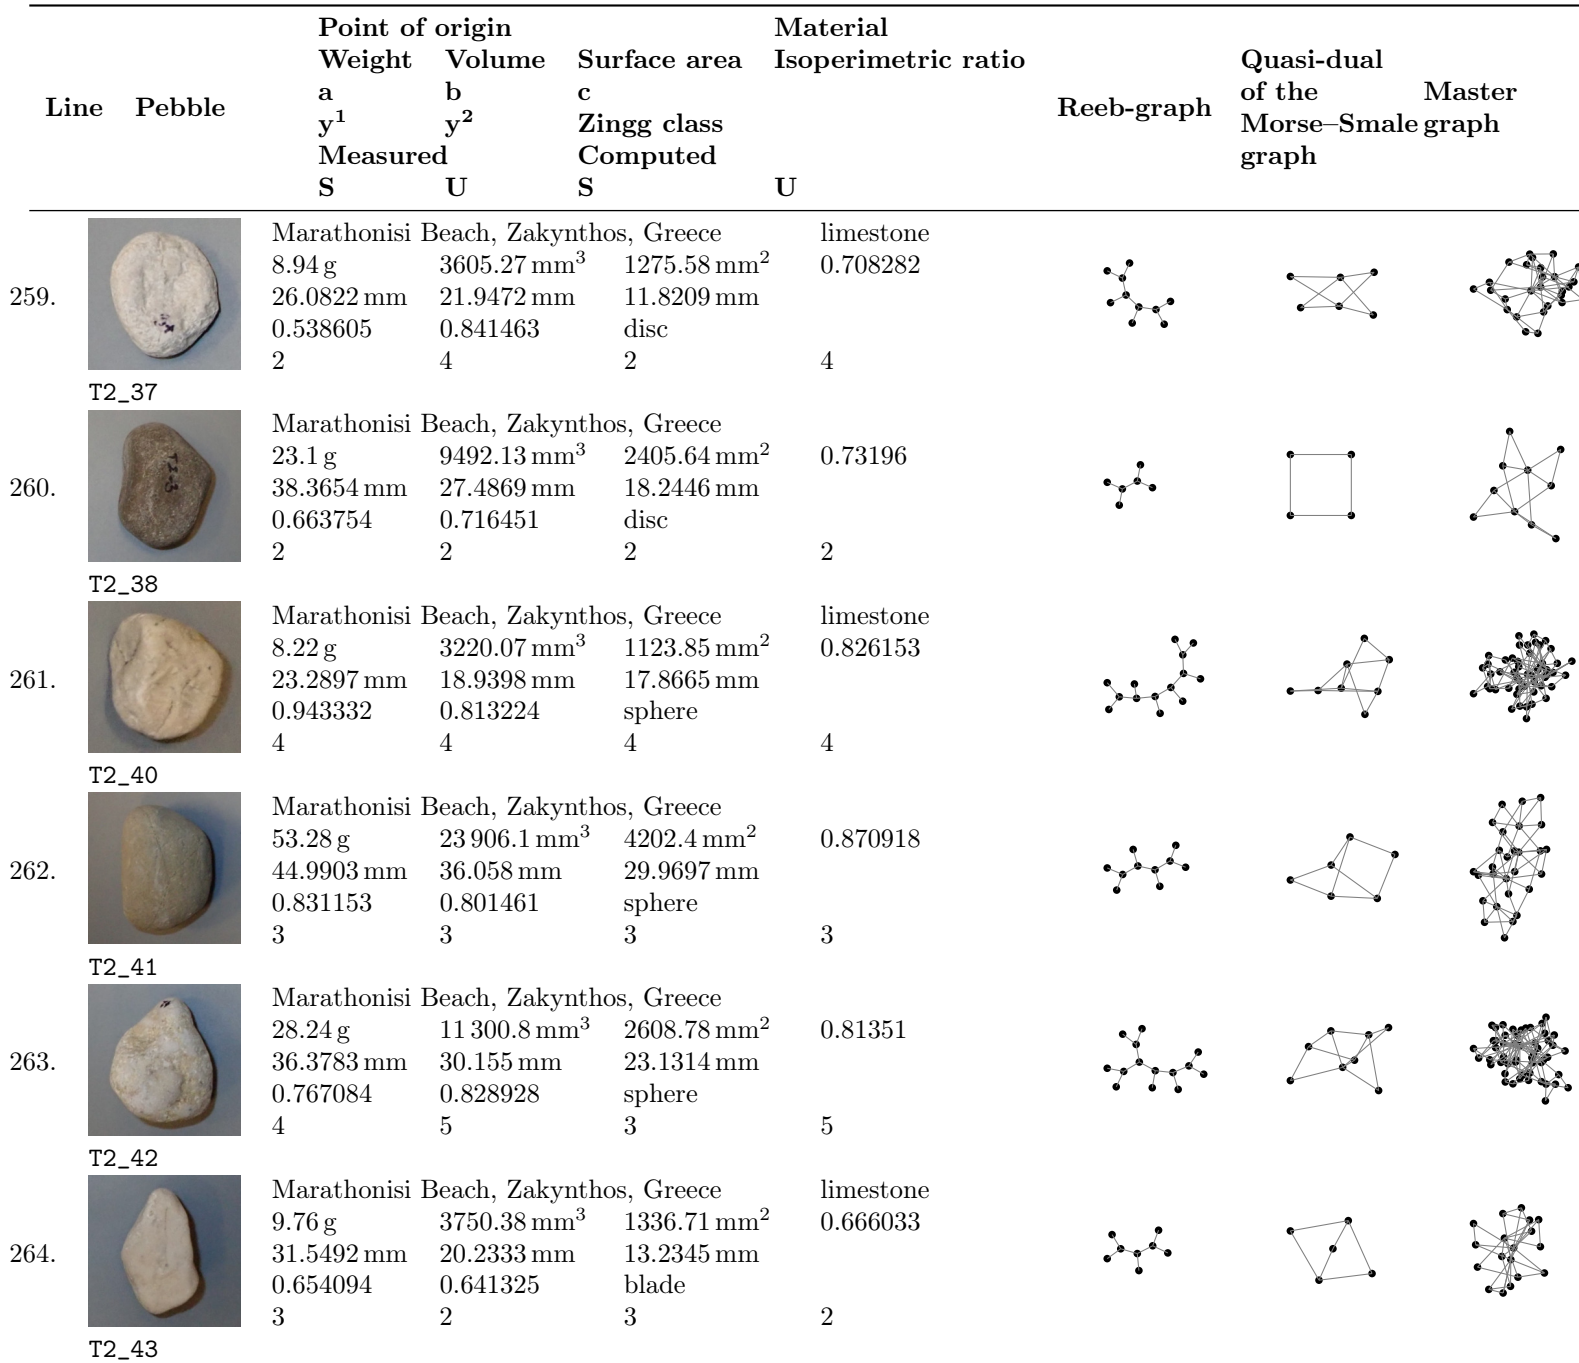   | Marathonisi Beach, Zakynthos, Greece<br>8.22 g<br>23.2897 mm<br>0.943332<br>4  | 3220.07 mm <sup>3</sup><br>18.9398 mm<br>0.813224<br>4 | 1123.85 mm <sup>2</sup><br>17.8665 mm<br>sphere<br>4 | limestone<br>0.826153<br><br>4 |                     | 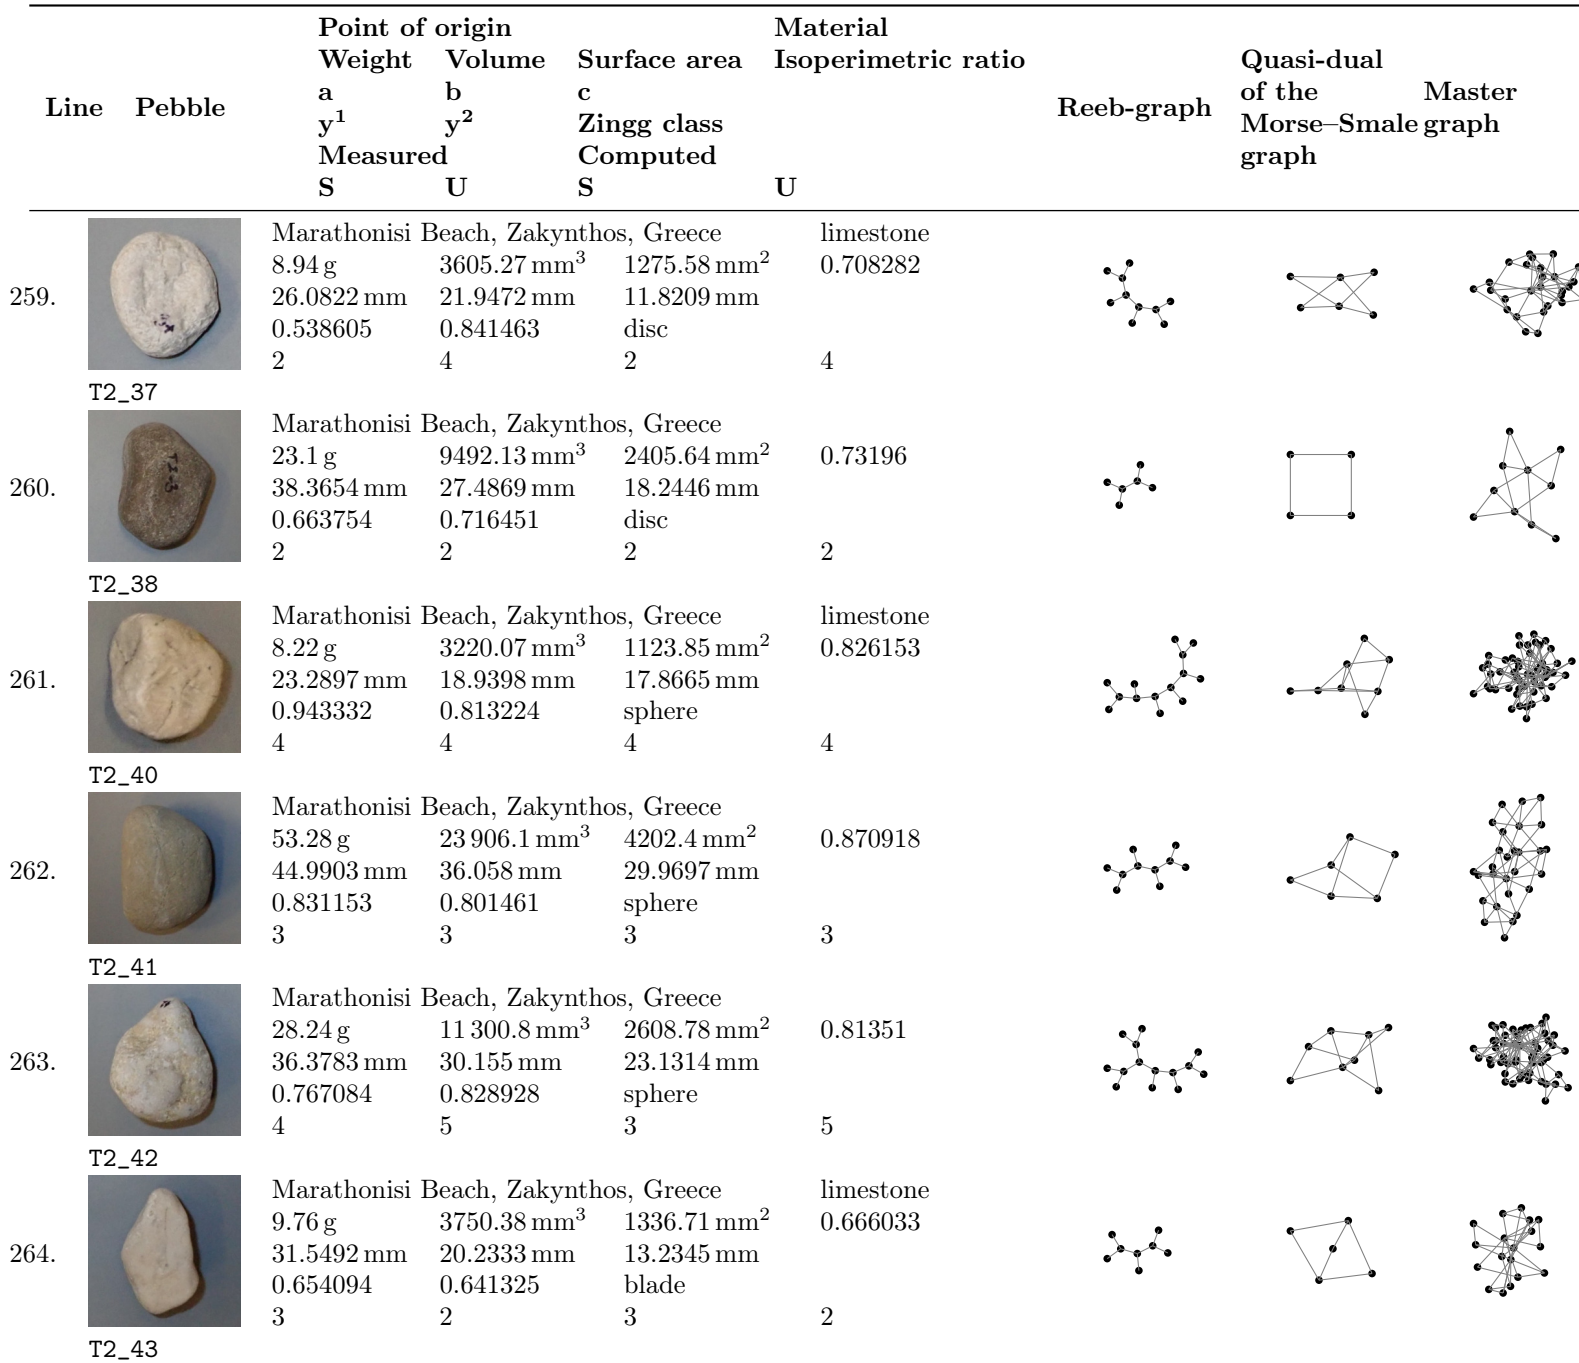   | 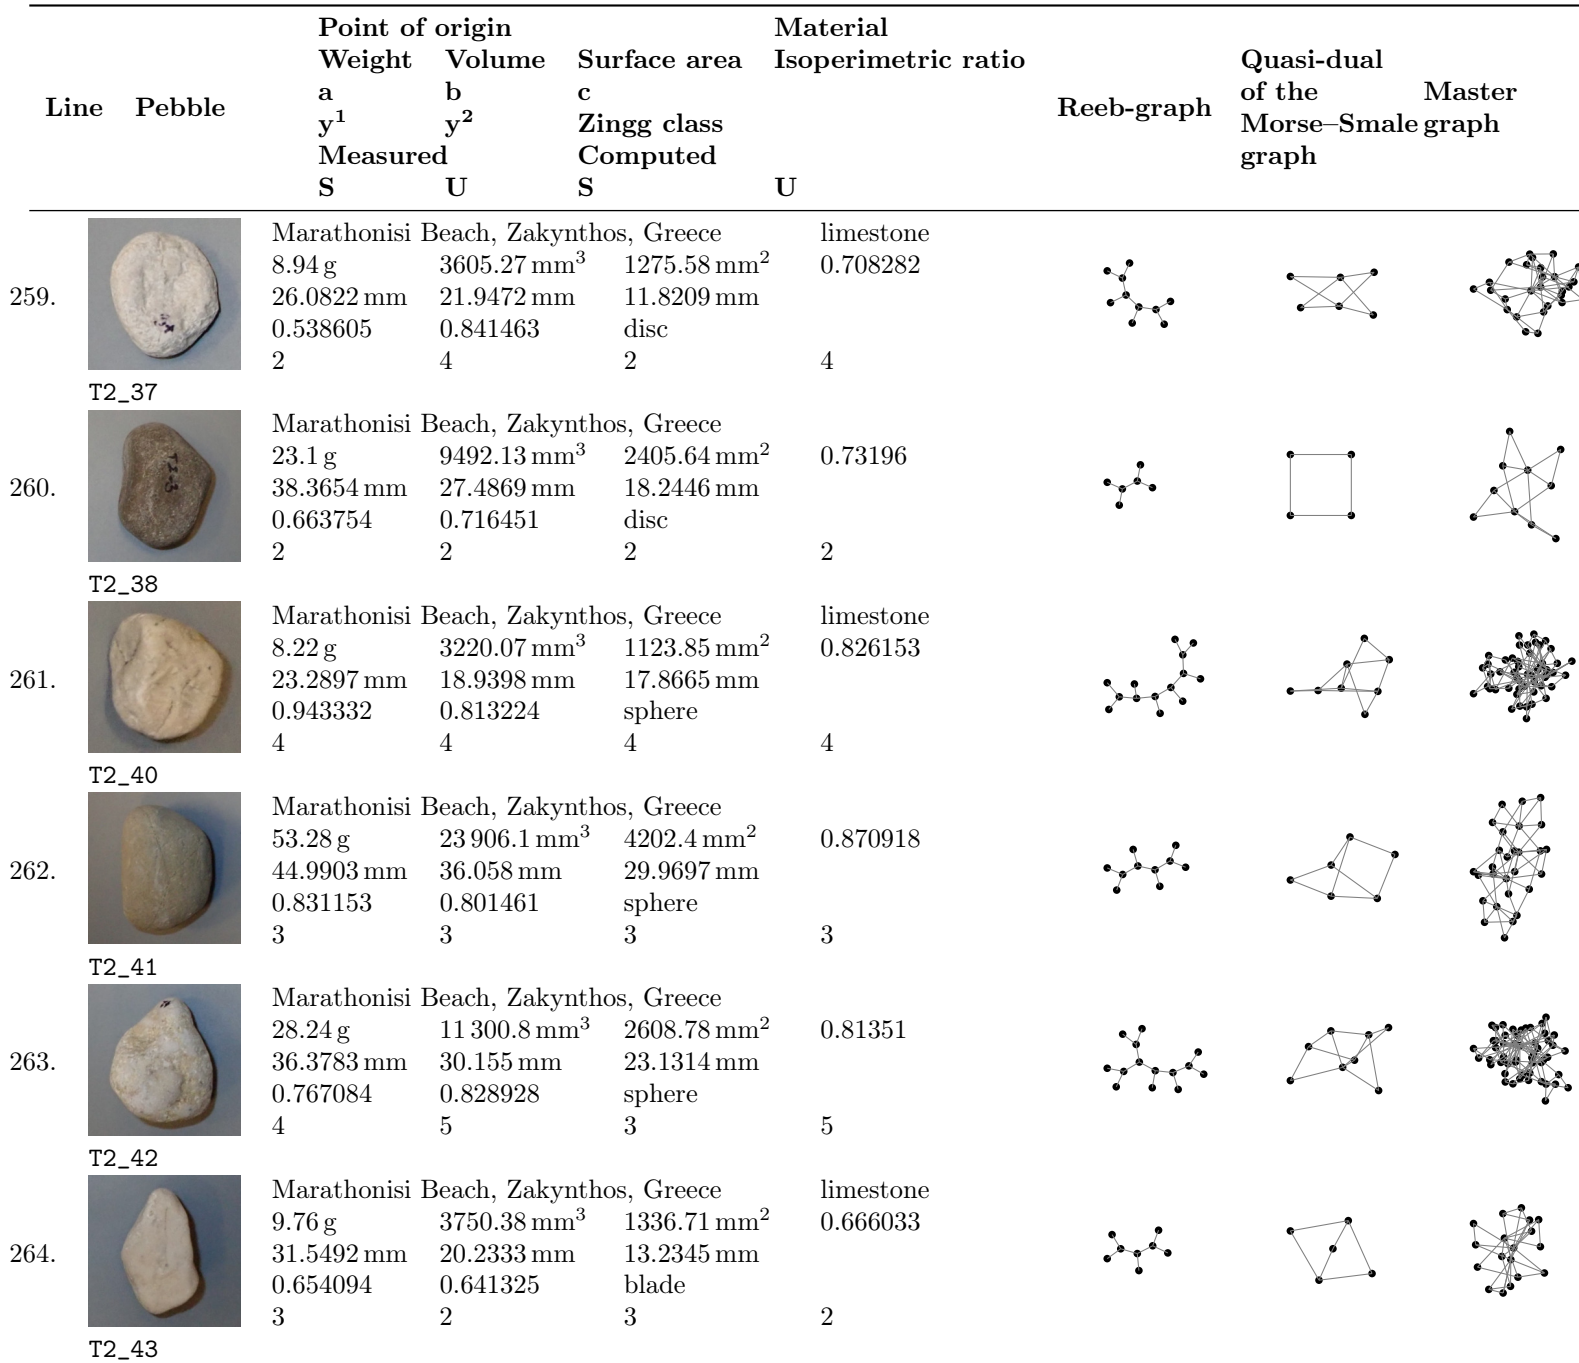   | 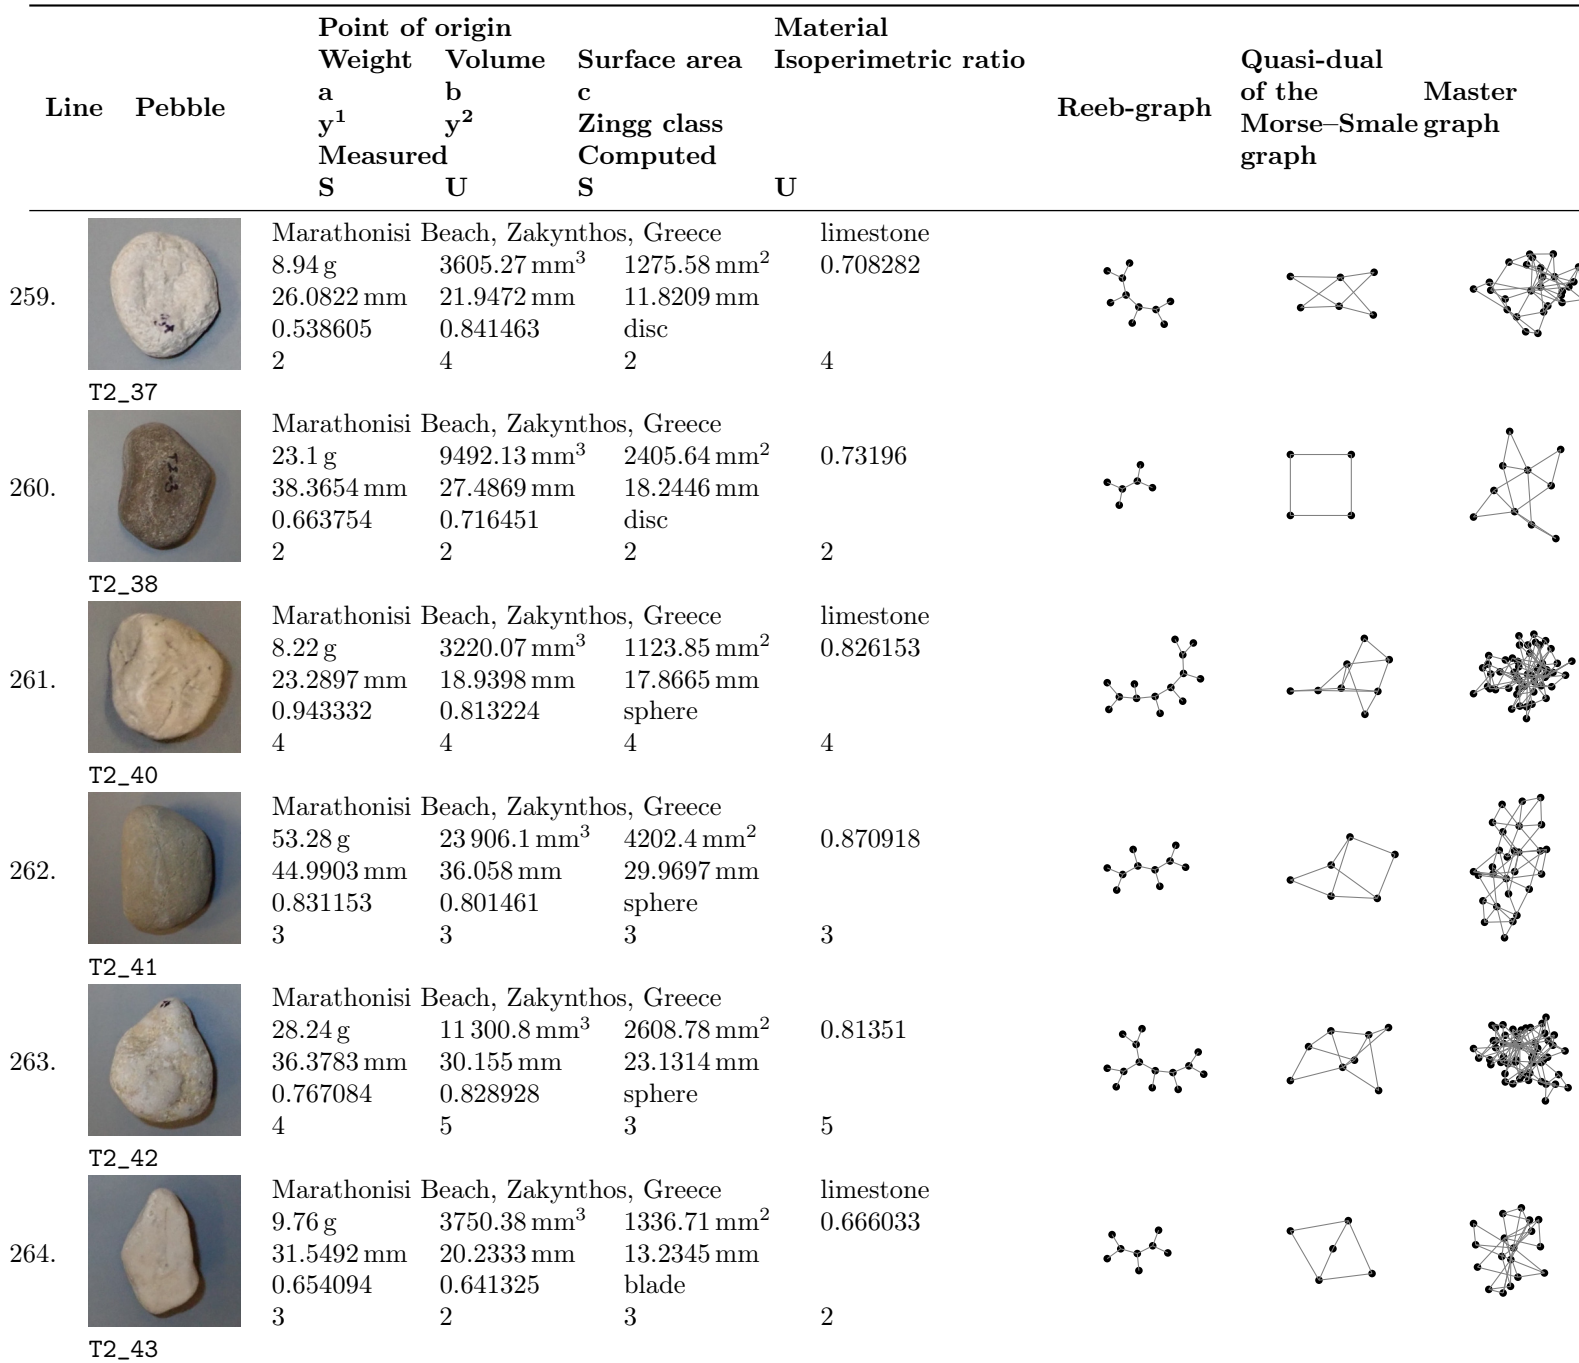   |
|      | T2_40                                                                               |                                                                                |                                                        |                                                      |                                |                     |                                                                                       |                                                                                       |                                                                                       |
| 262. | 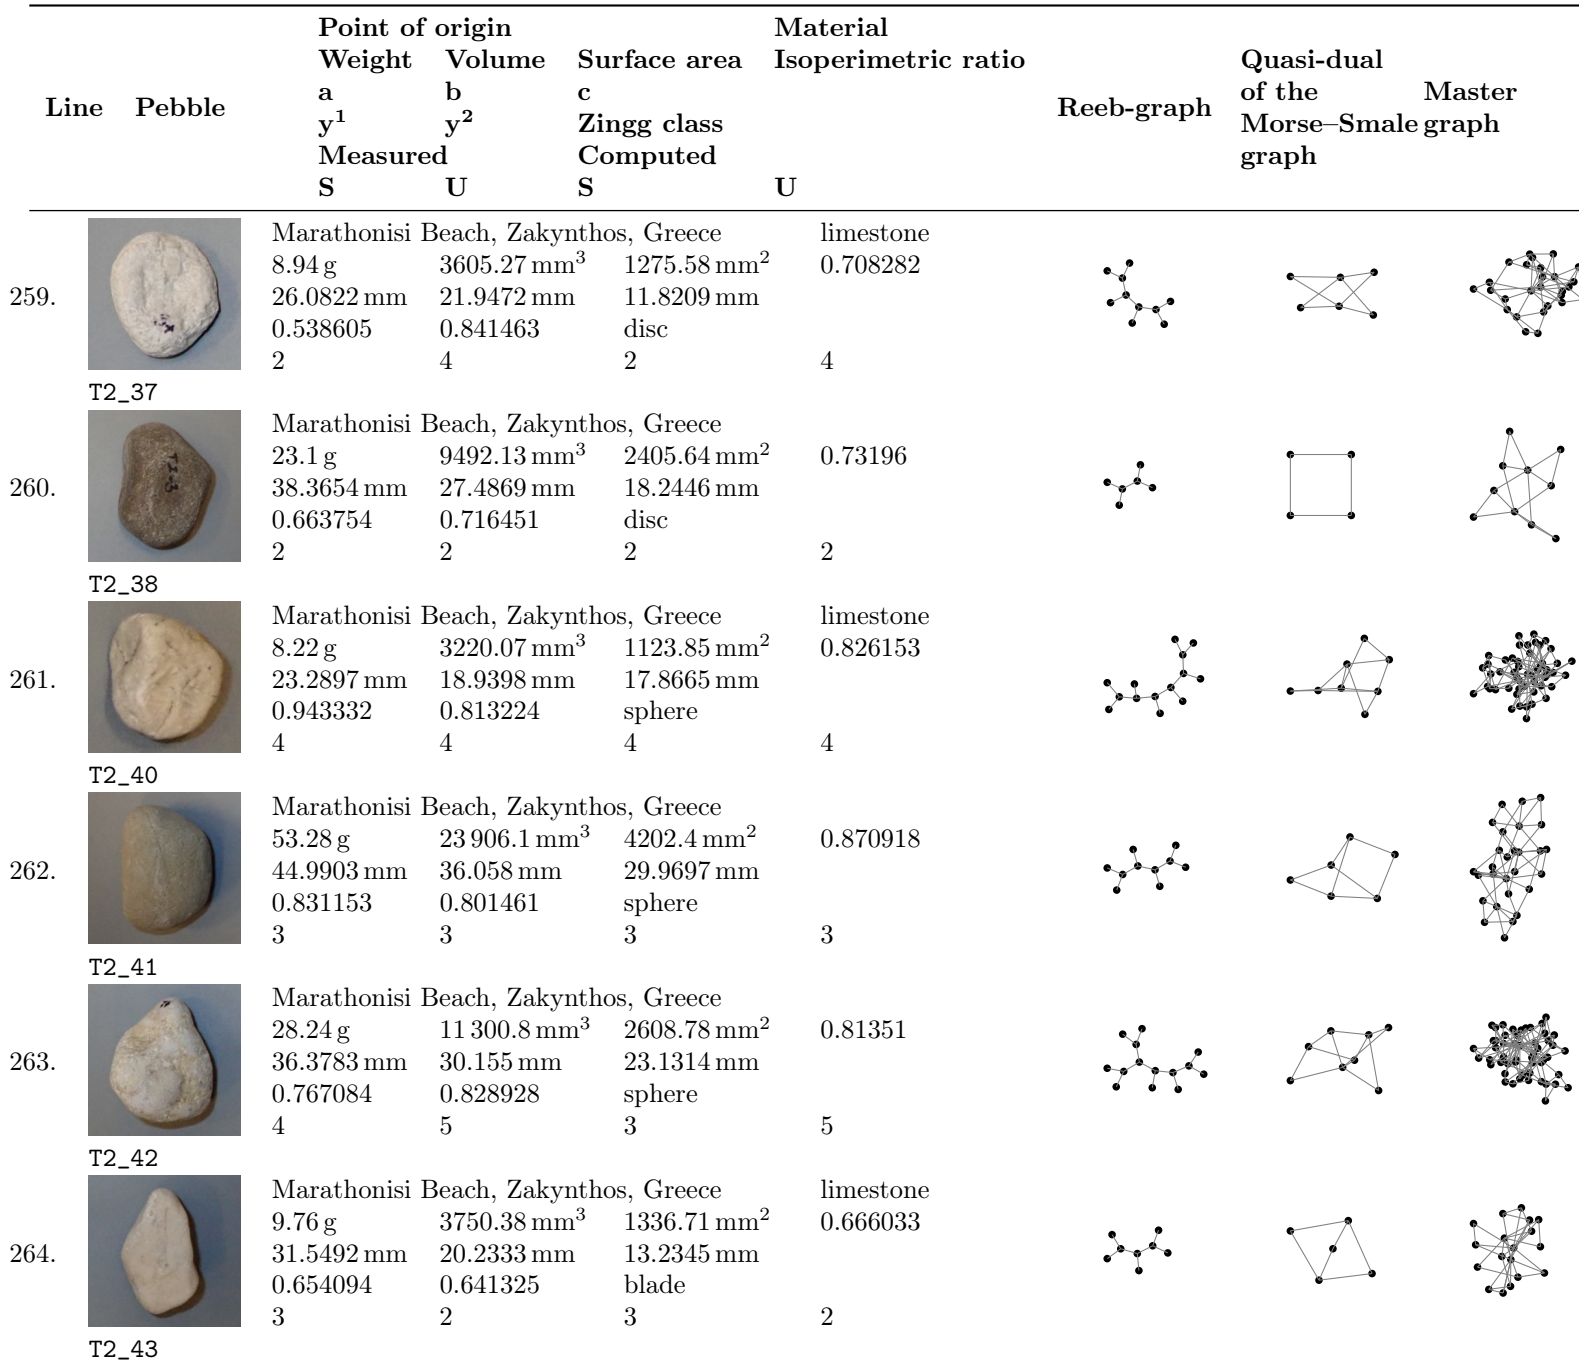  | Marathonisi Beach, Zakynthos, Greece<br>53.28 g<br>44.9903 mm<br>0.831153<br>3 | 23 906.1 mm <sup>3</sup><br>36.058 mm<br>0.801461<br>3 | 4202.4 mm <sup>2</sup><br>29.9697 mm<br>sphere<br>3  | 0.870918<br><br>3              |                     | 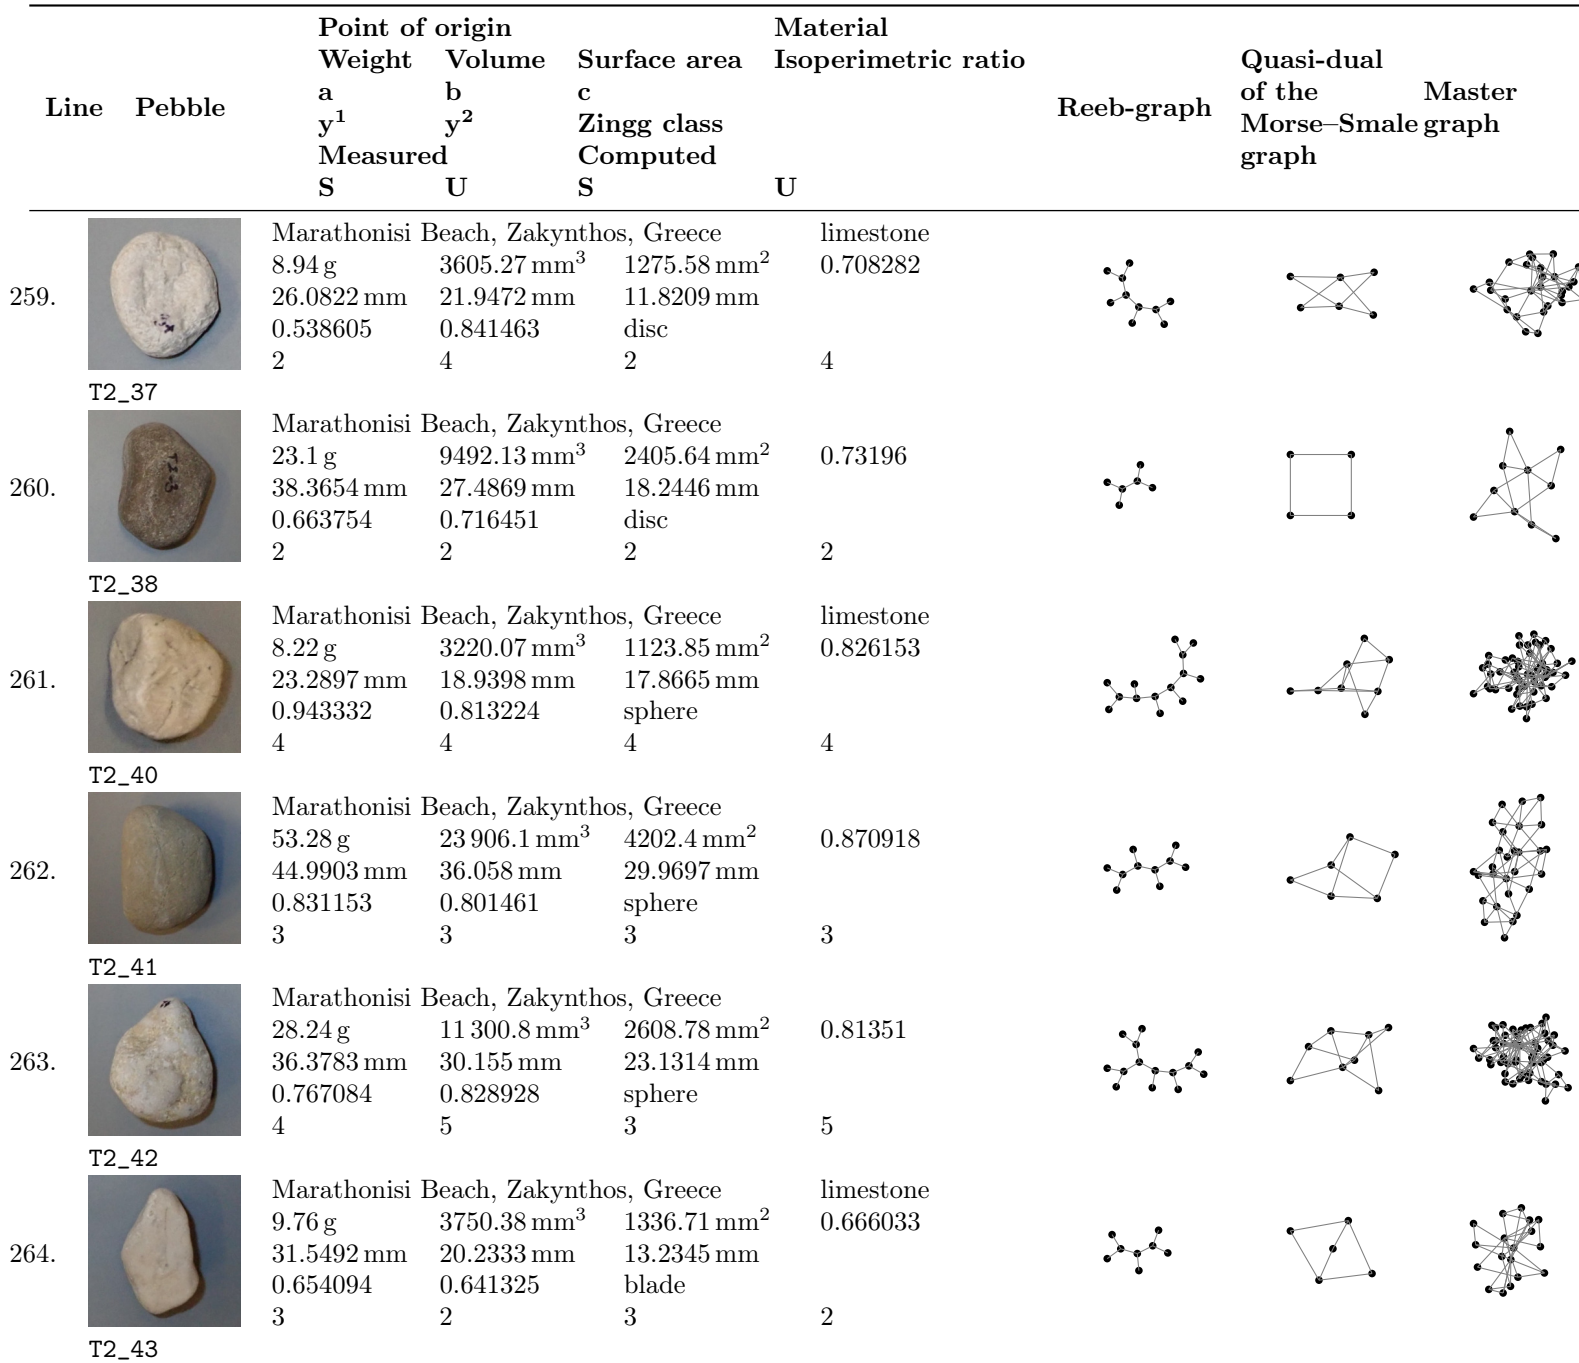  | 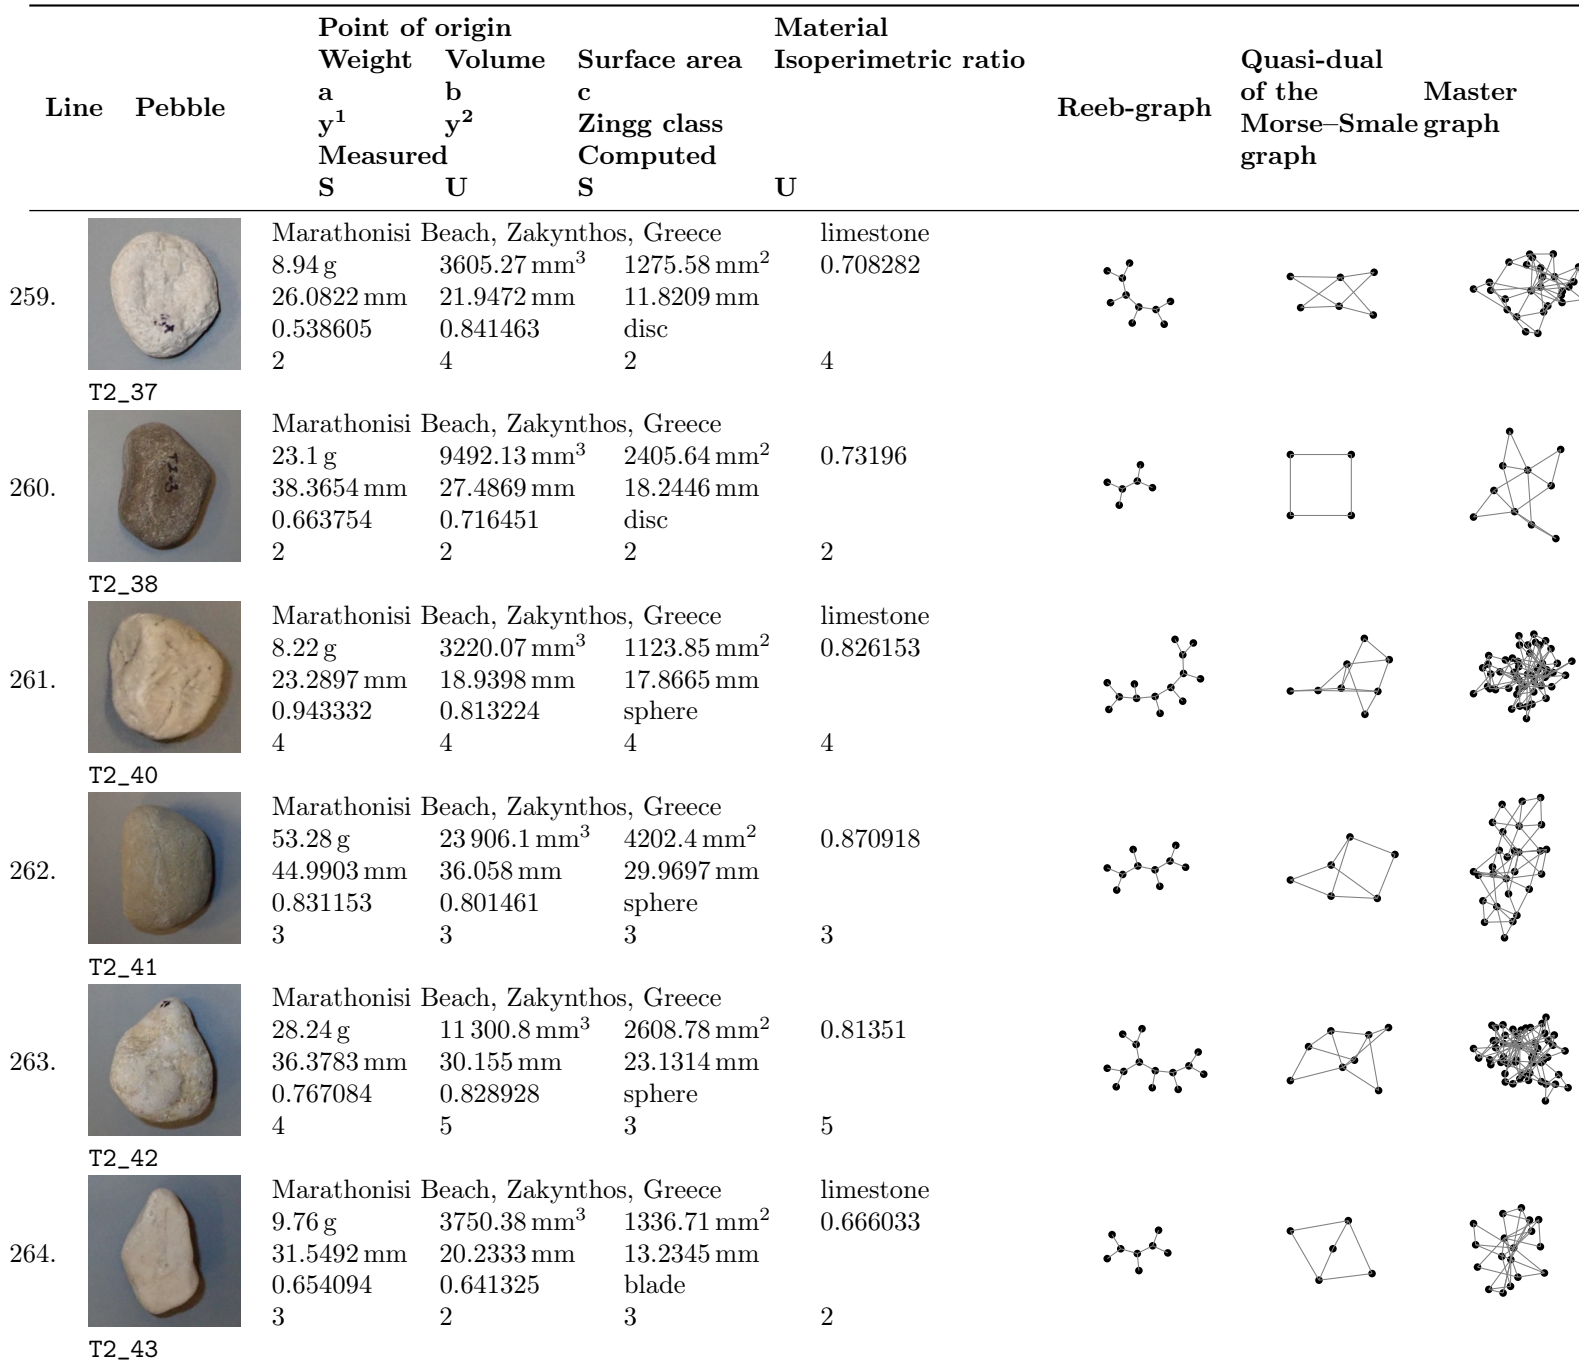  | 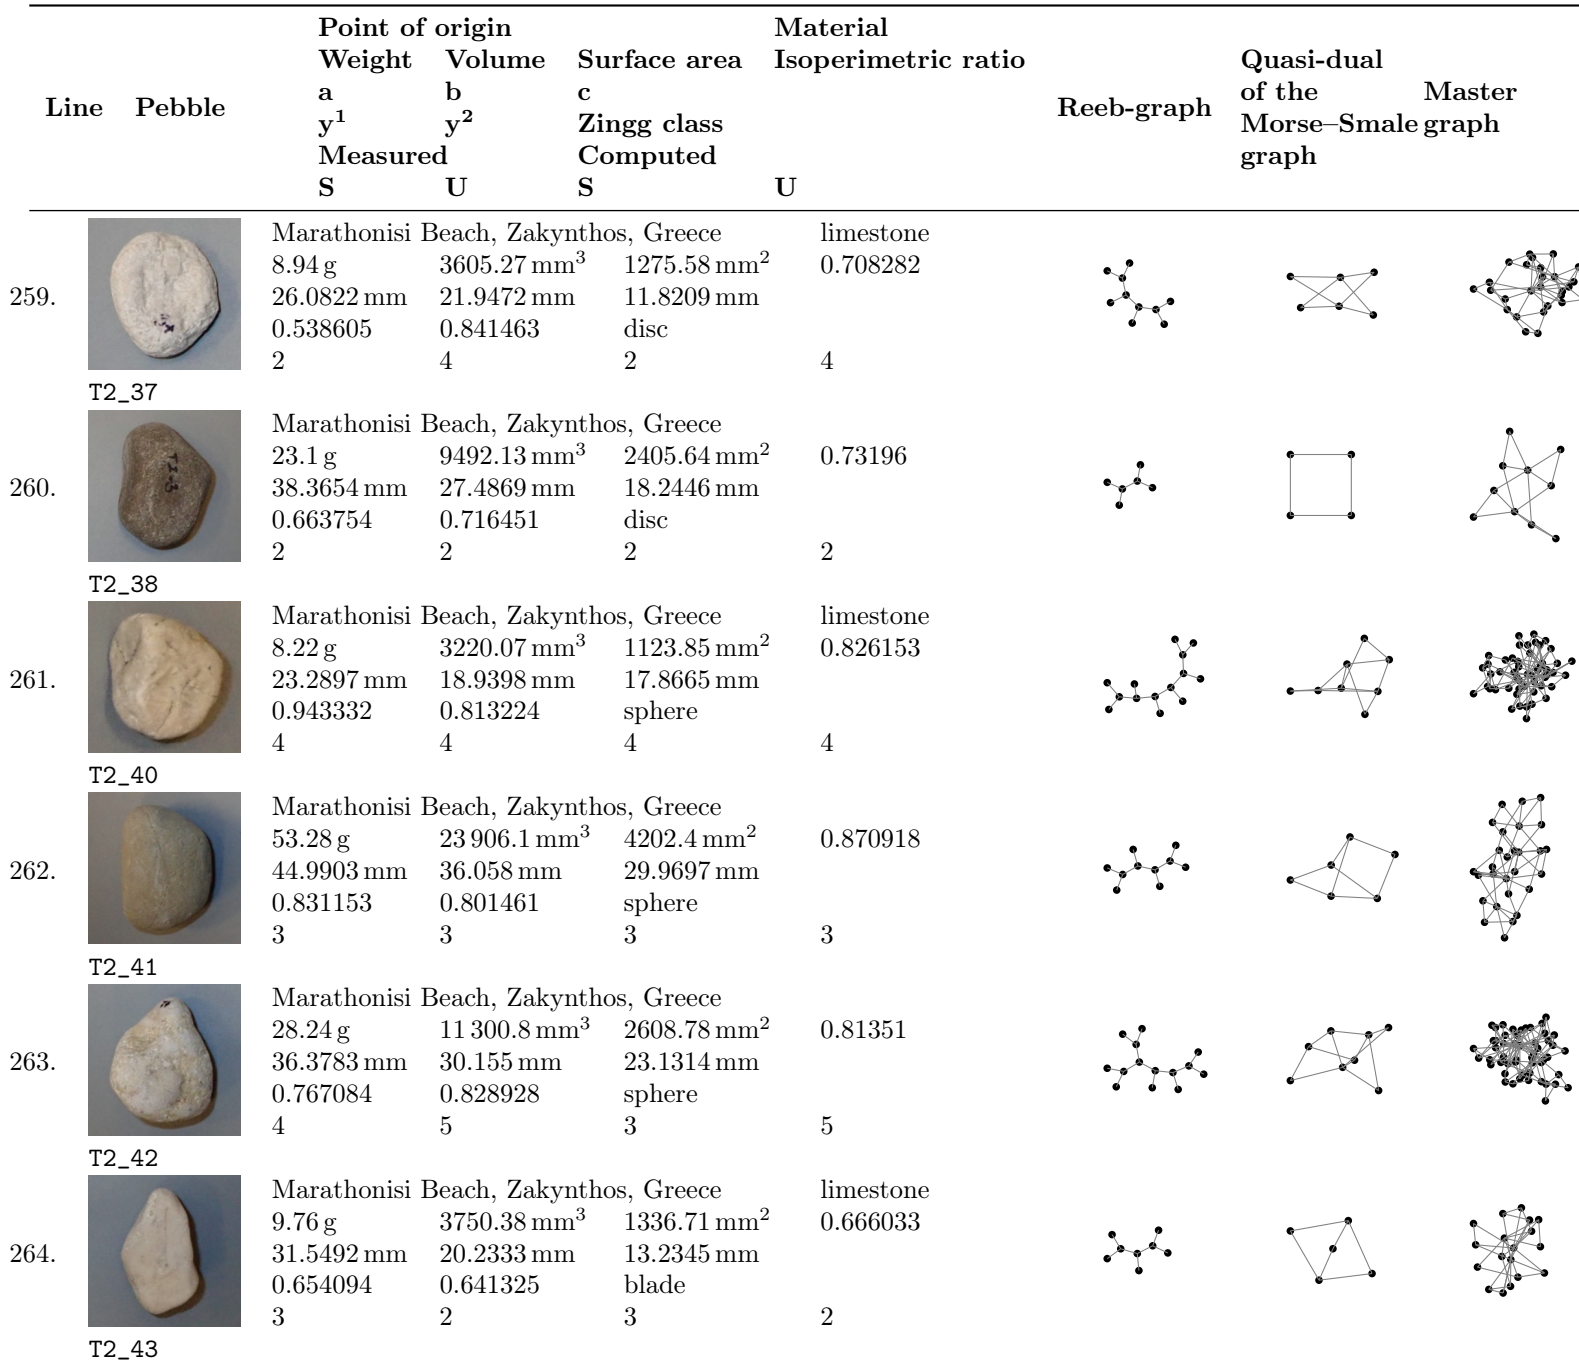  |
|      | T2_41                                                                               |                                                                                |                                                        |                                                      |                                |                     |                                                                                       |                                                                                       |                                                                                       |
| 263. | 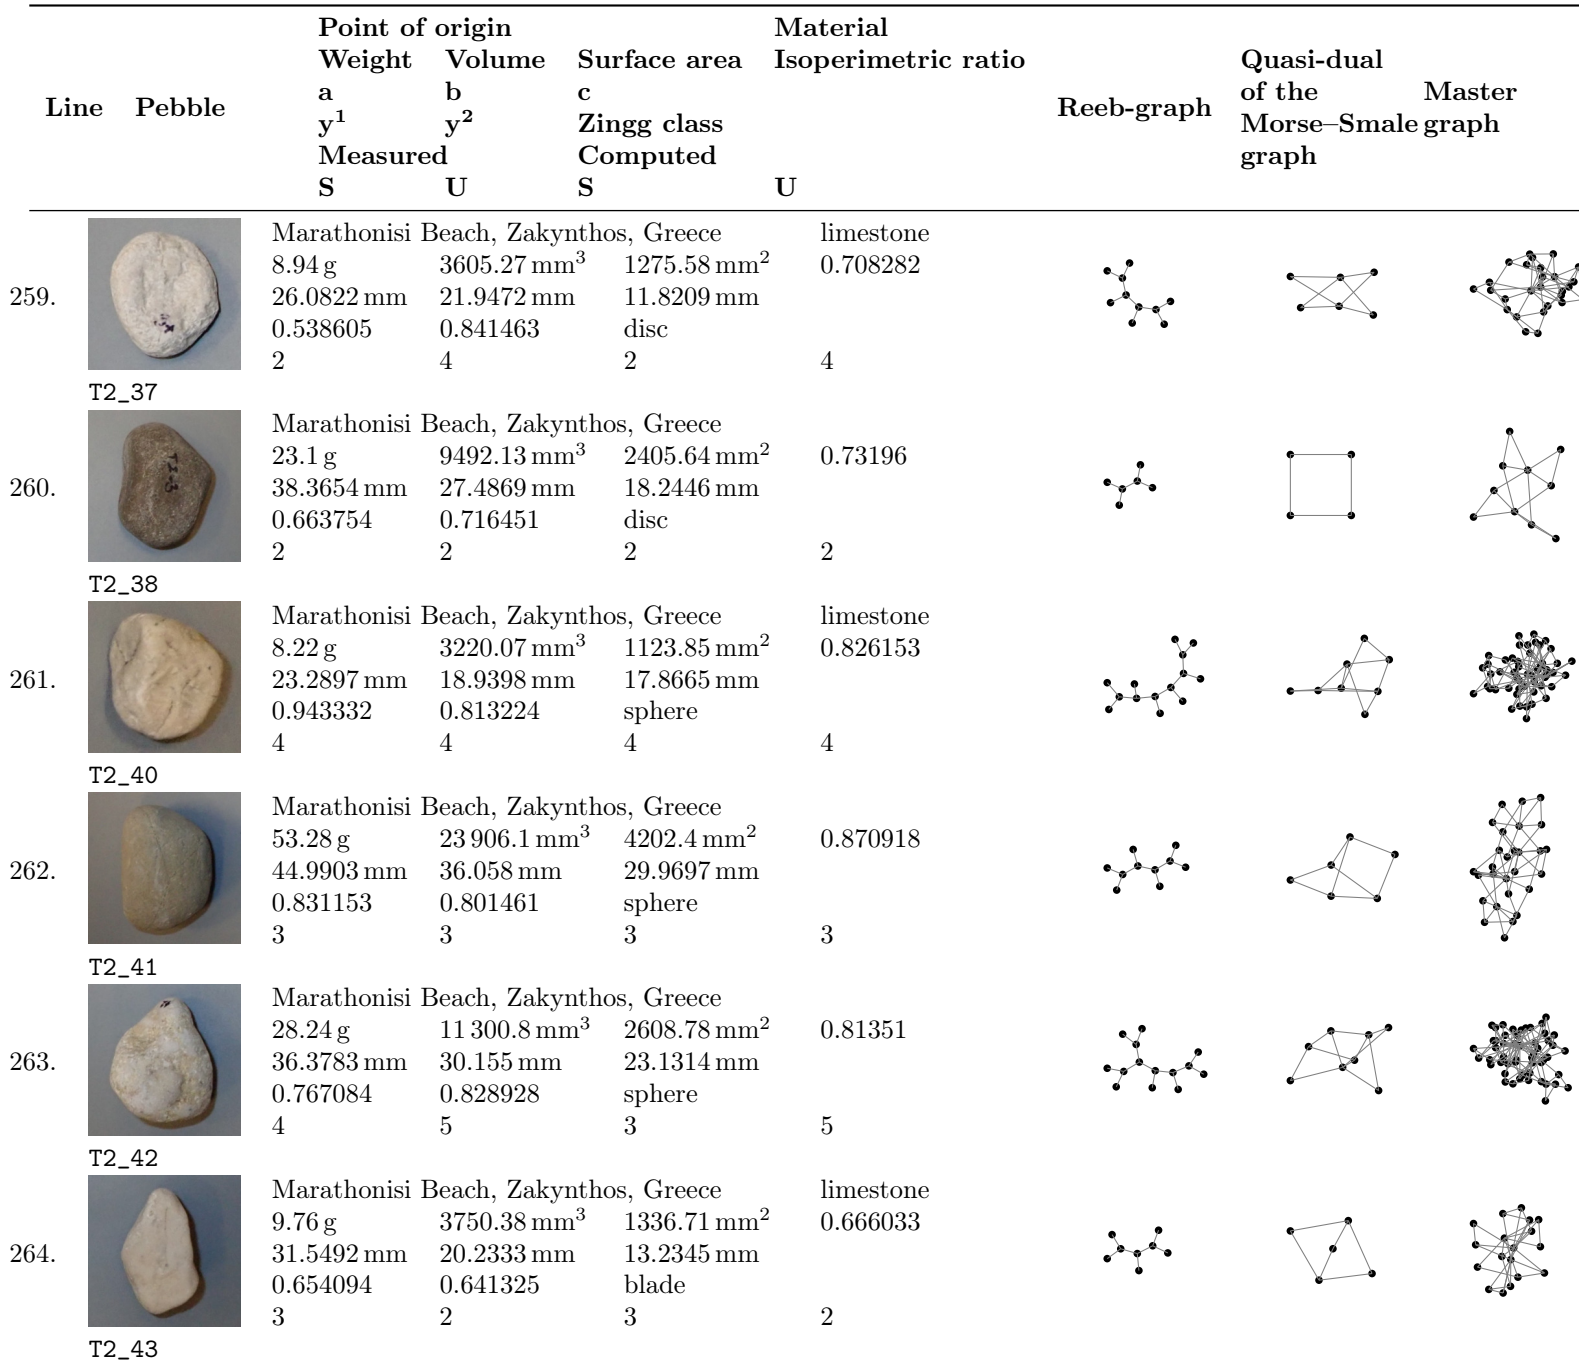 | Marathonisi Beach, Zakynthos, Greece<br>28.24 g<br>36.3783 mm<br>0.767084<br>4 | 11 300.8 mm <sup>3</sup><br>30.155 mm<br>0.828928<br>5 | 2608.78 mm <sup>2</sup><br>23.1314 mm<br>sphere<br>3 | 0.81351<br><br>5               |                     | 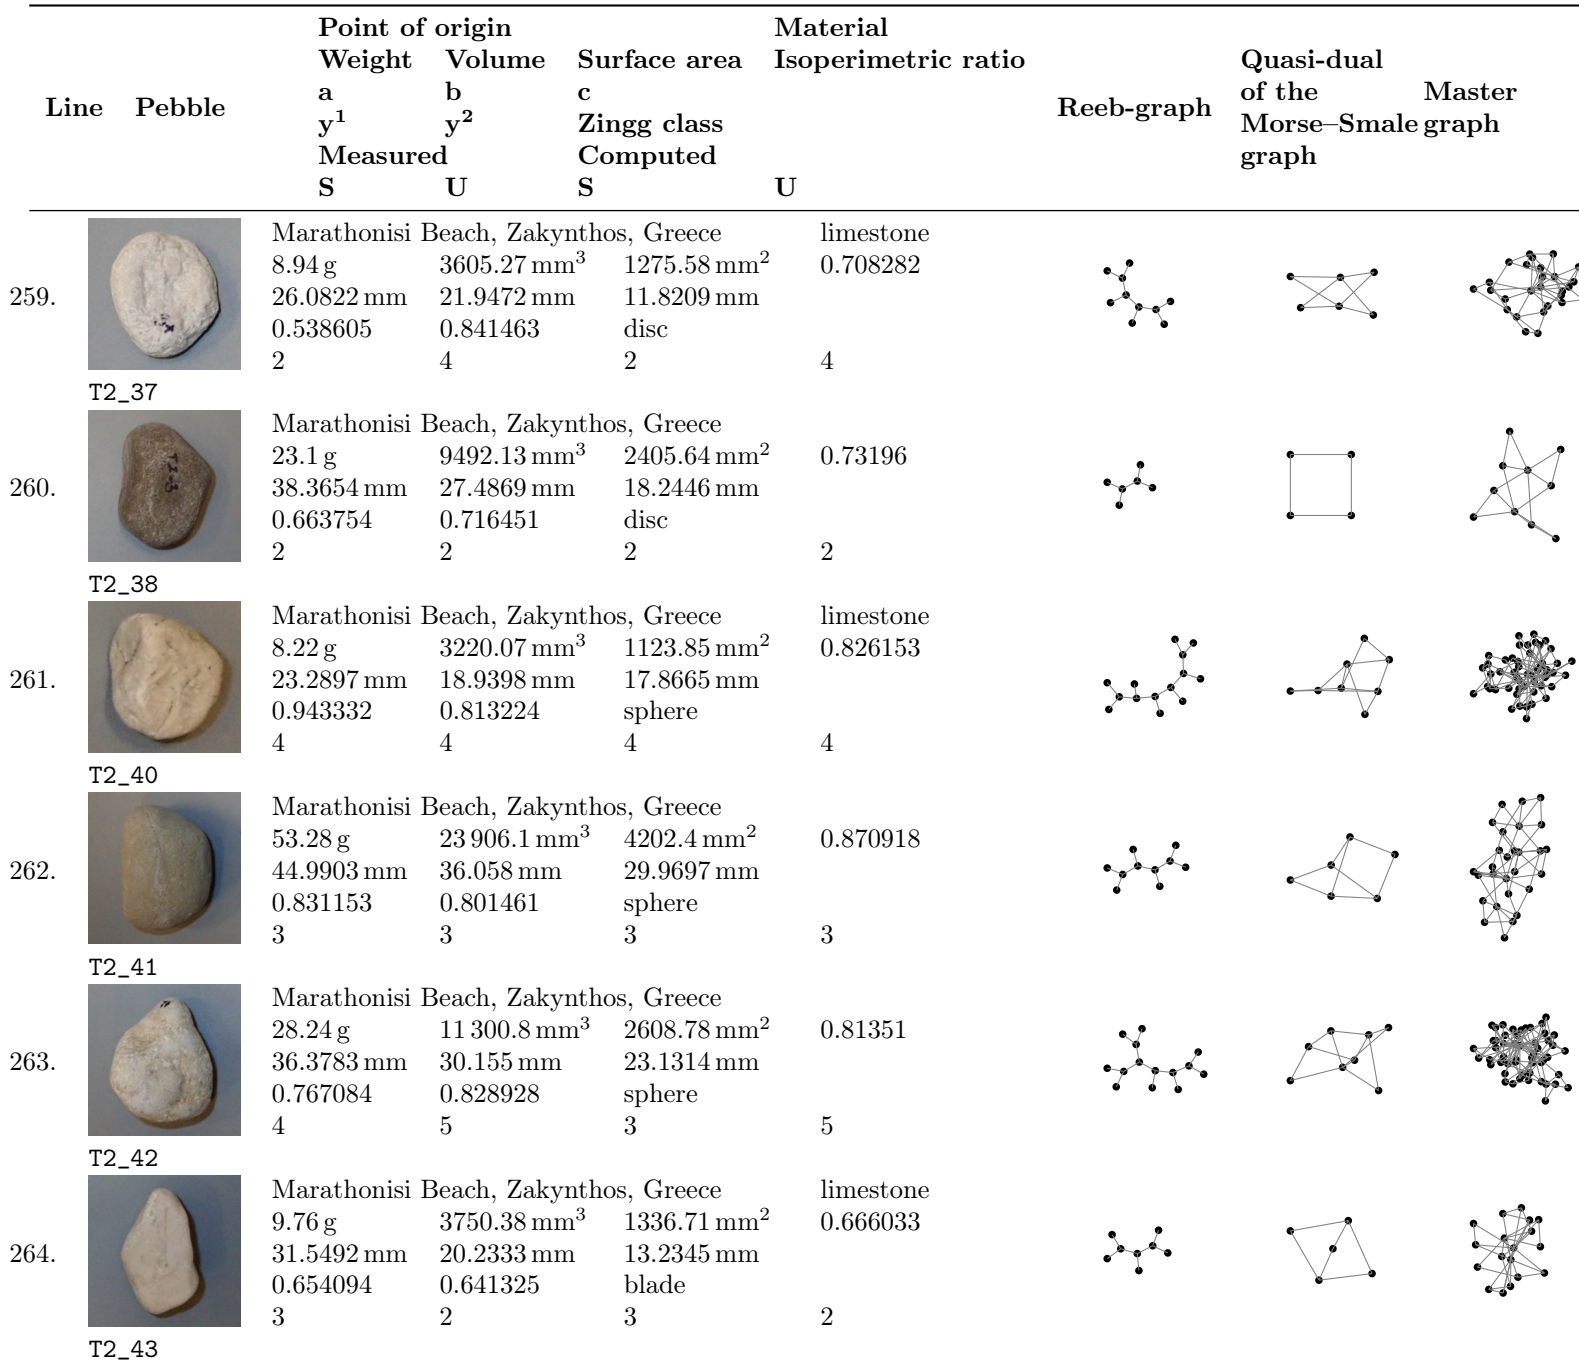 | 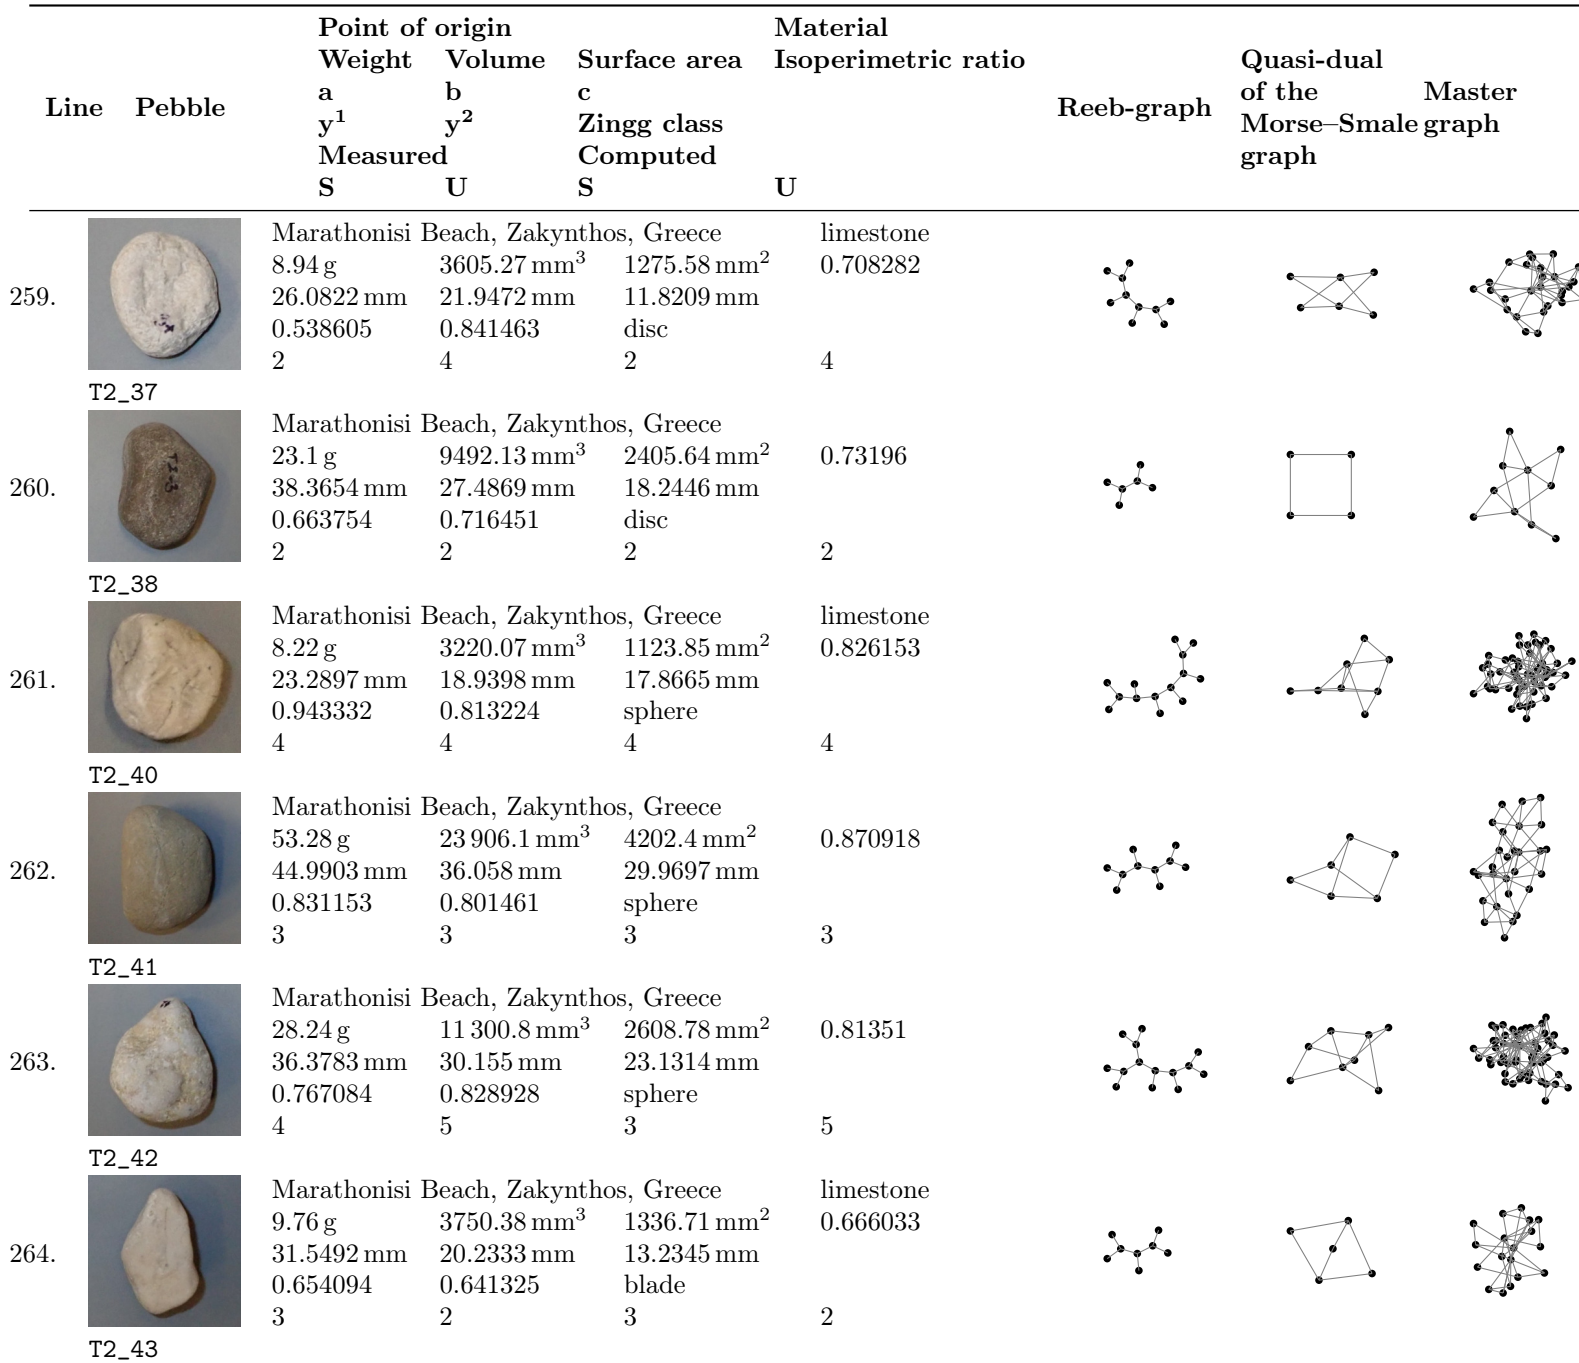 | 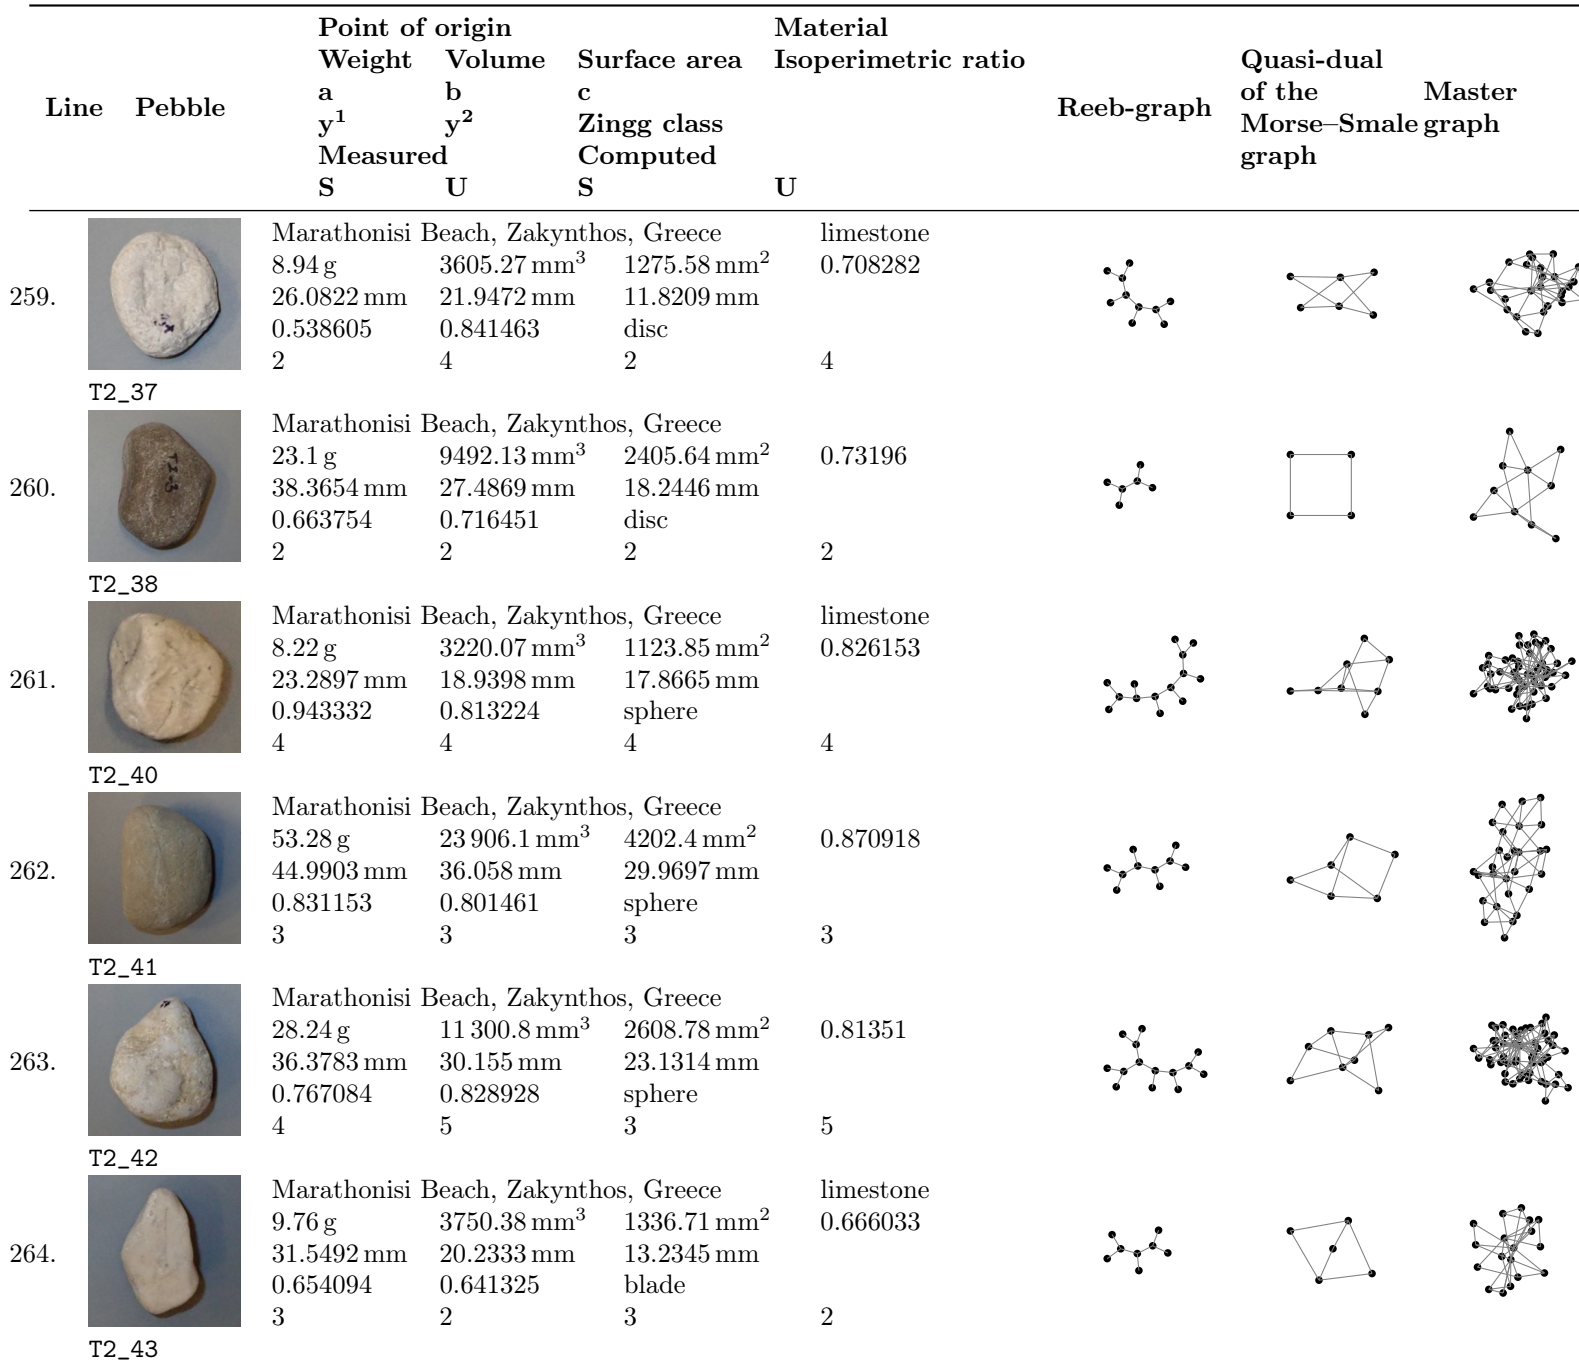 |
|      | T2_42                                                                               |                                                                                |                                                        |                                                      |                                |                     |                                                                                       |                                                                                       |                                                                                       |
| 264. | 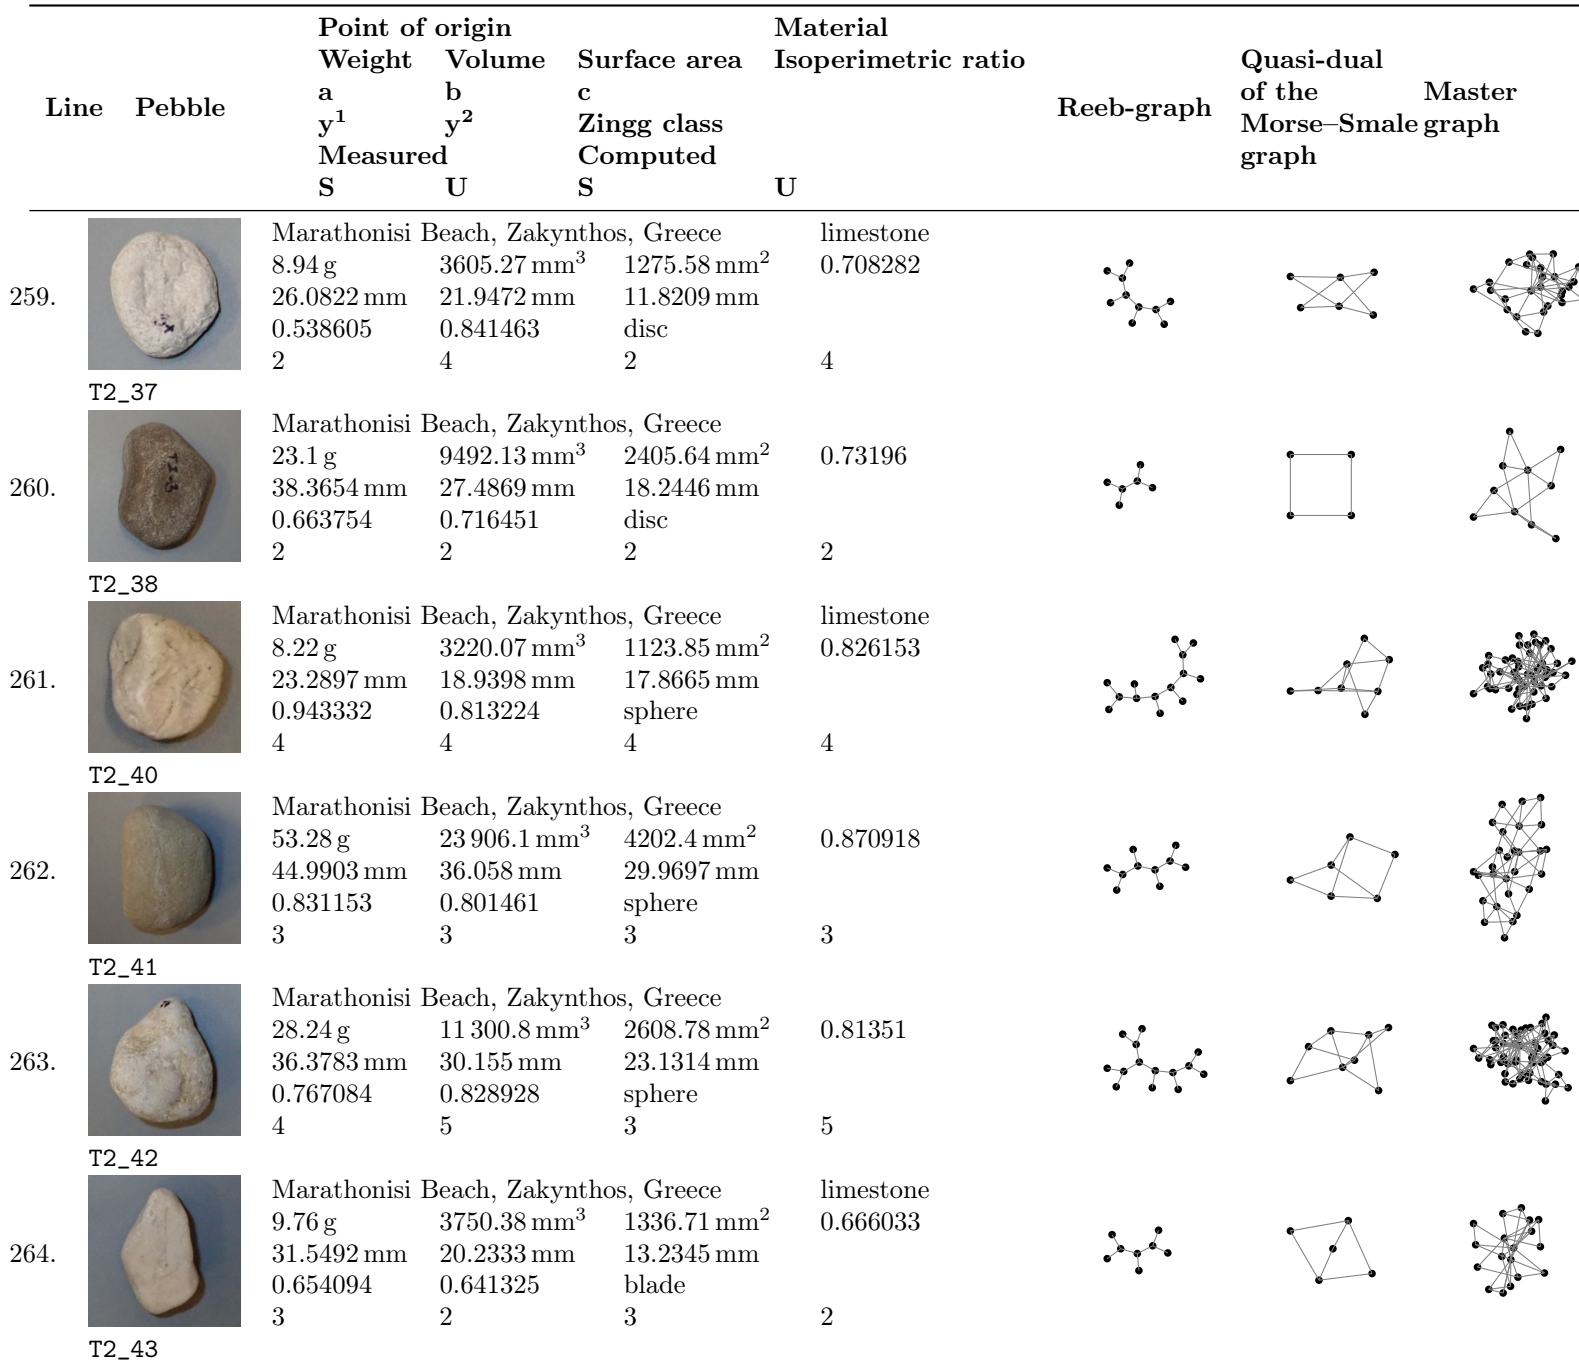 | Marathonisi Beach, Zakynthos, Greece<br>9.76 g<br>31.5492 mm<br>0.654094<br>3  | 3750.38 mm <sup>3</sup><br>20.2333 mm<br>0.641325<br>2 | 1336.71 mm <sup>2</sup><br>13.2345 mm<br>blade<br>3  | limestone<br>0.666033<br><br>2 |                     | 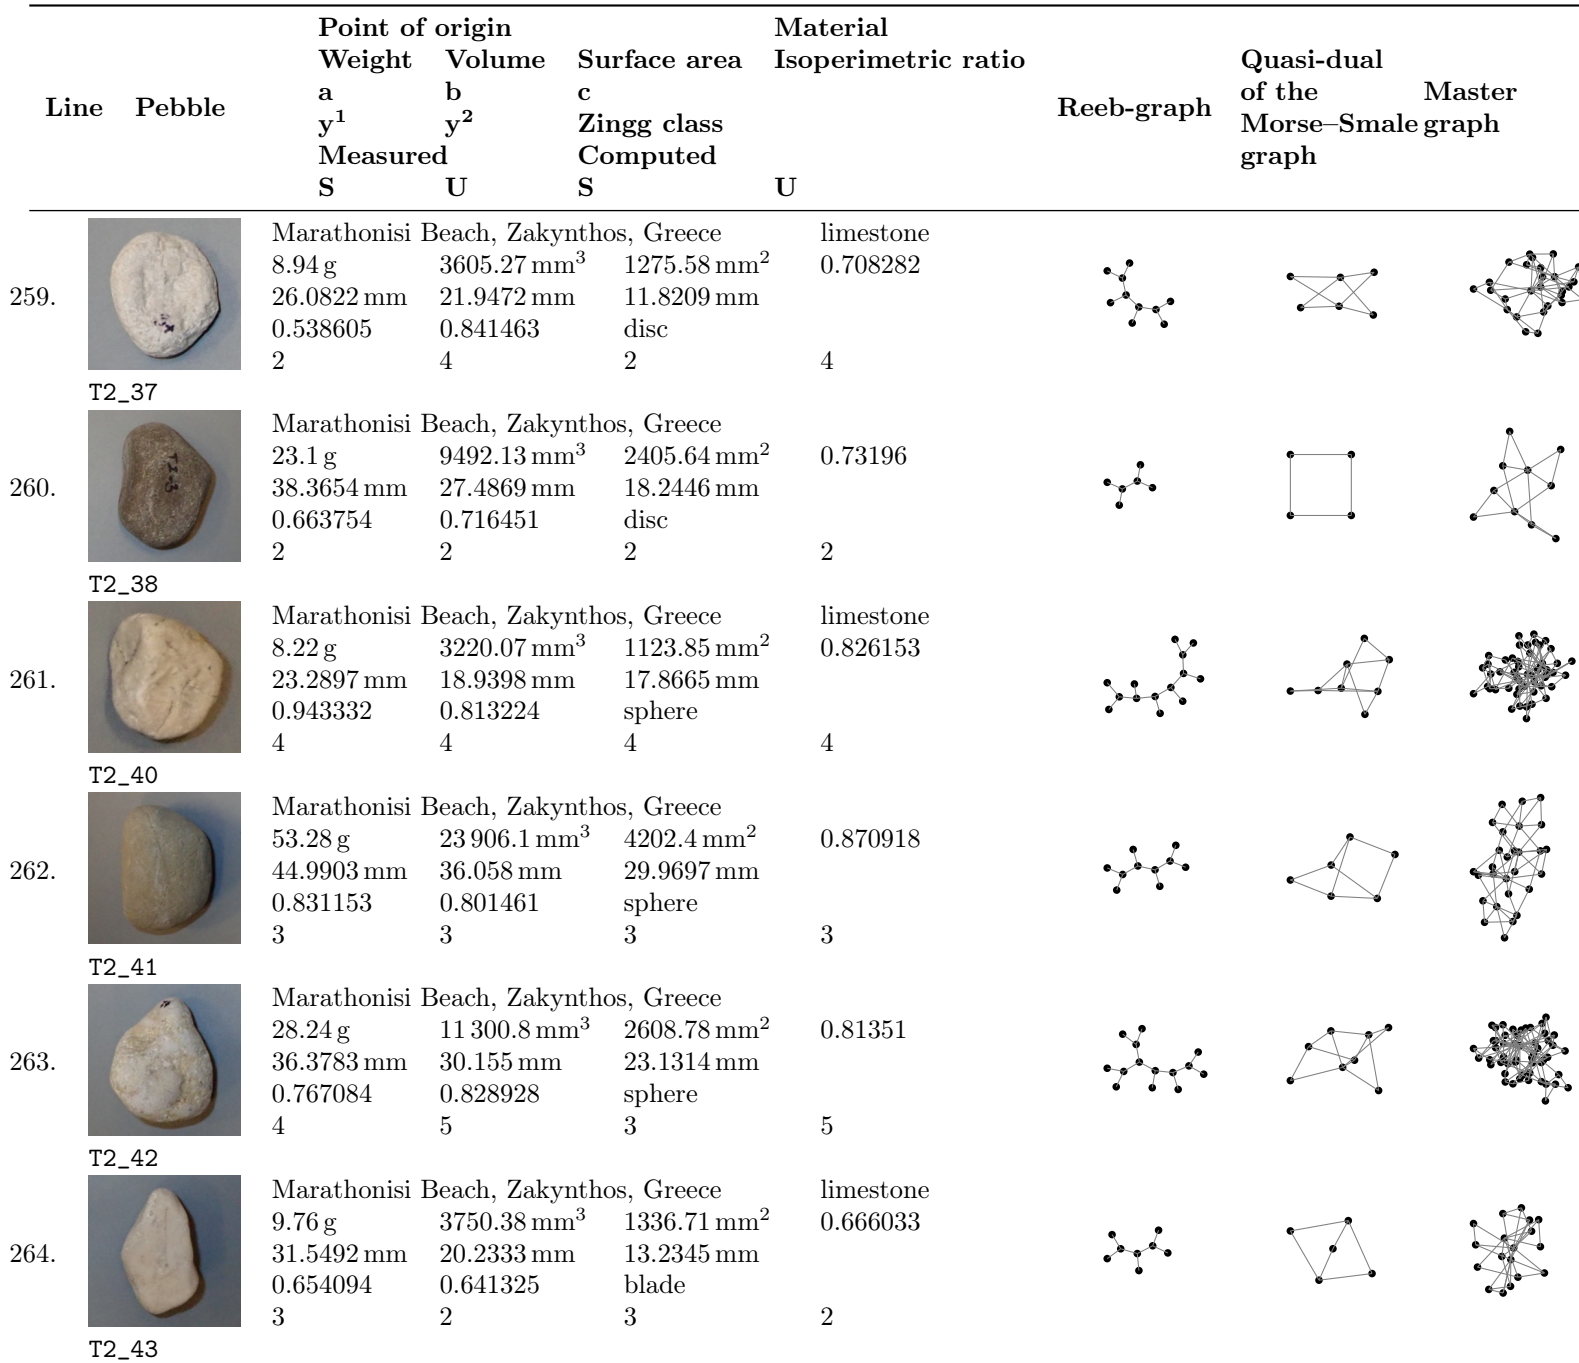 | 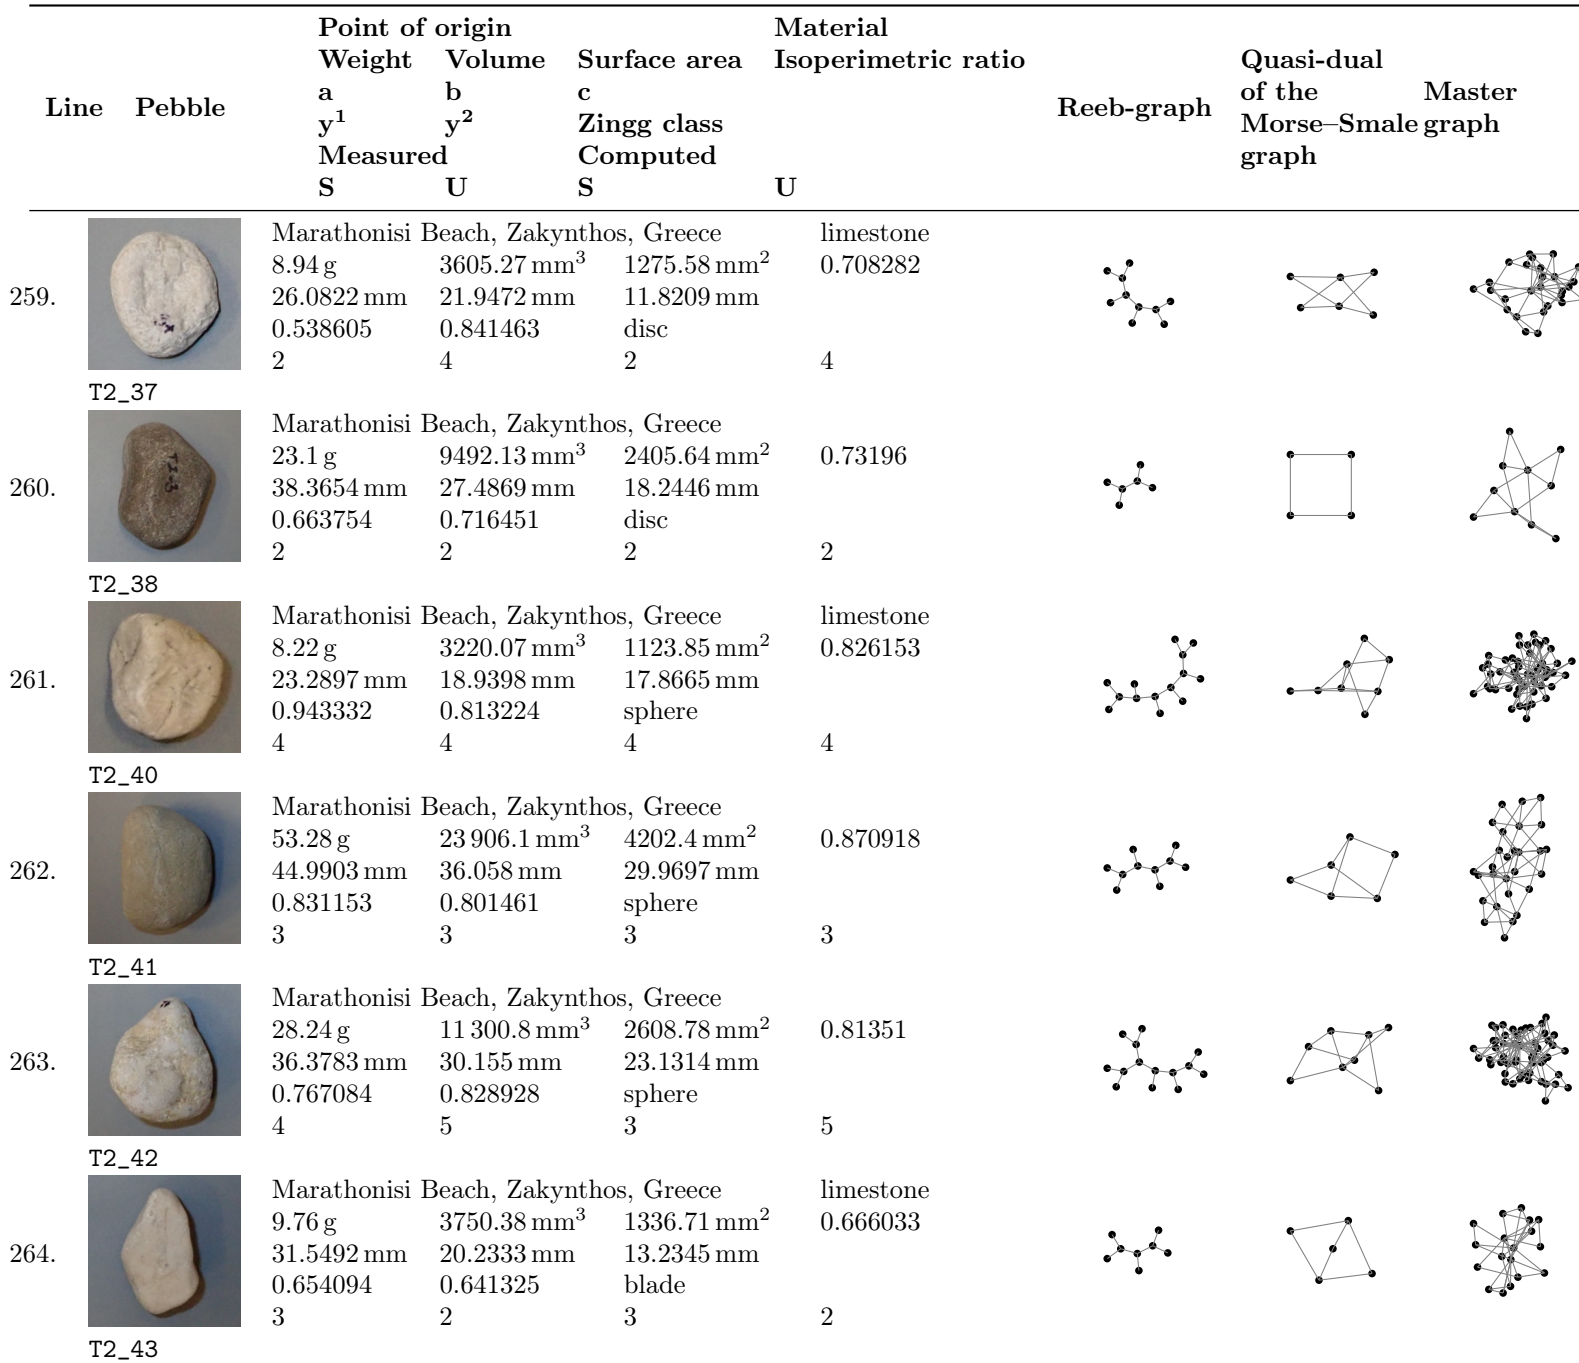 | 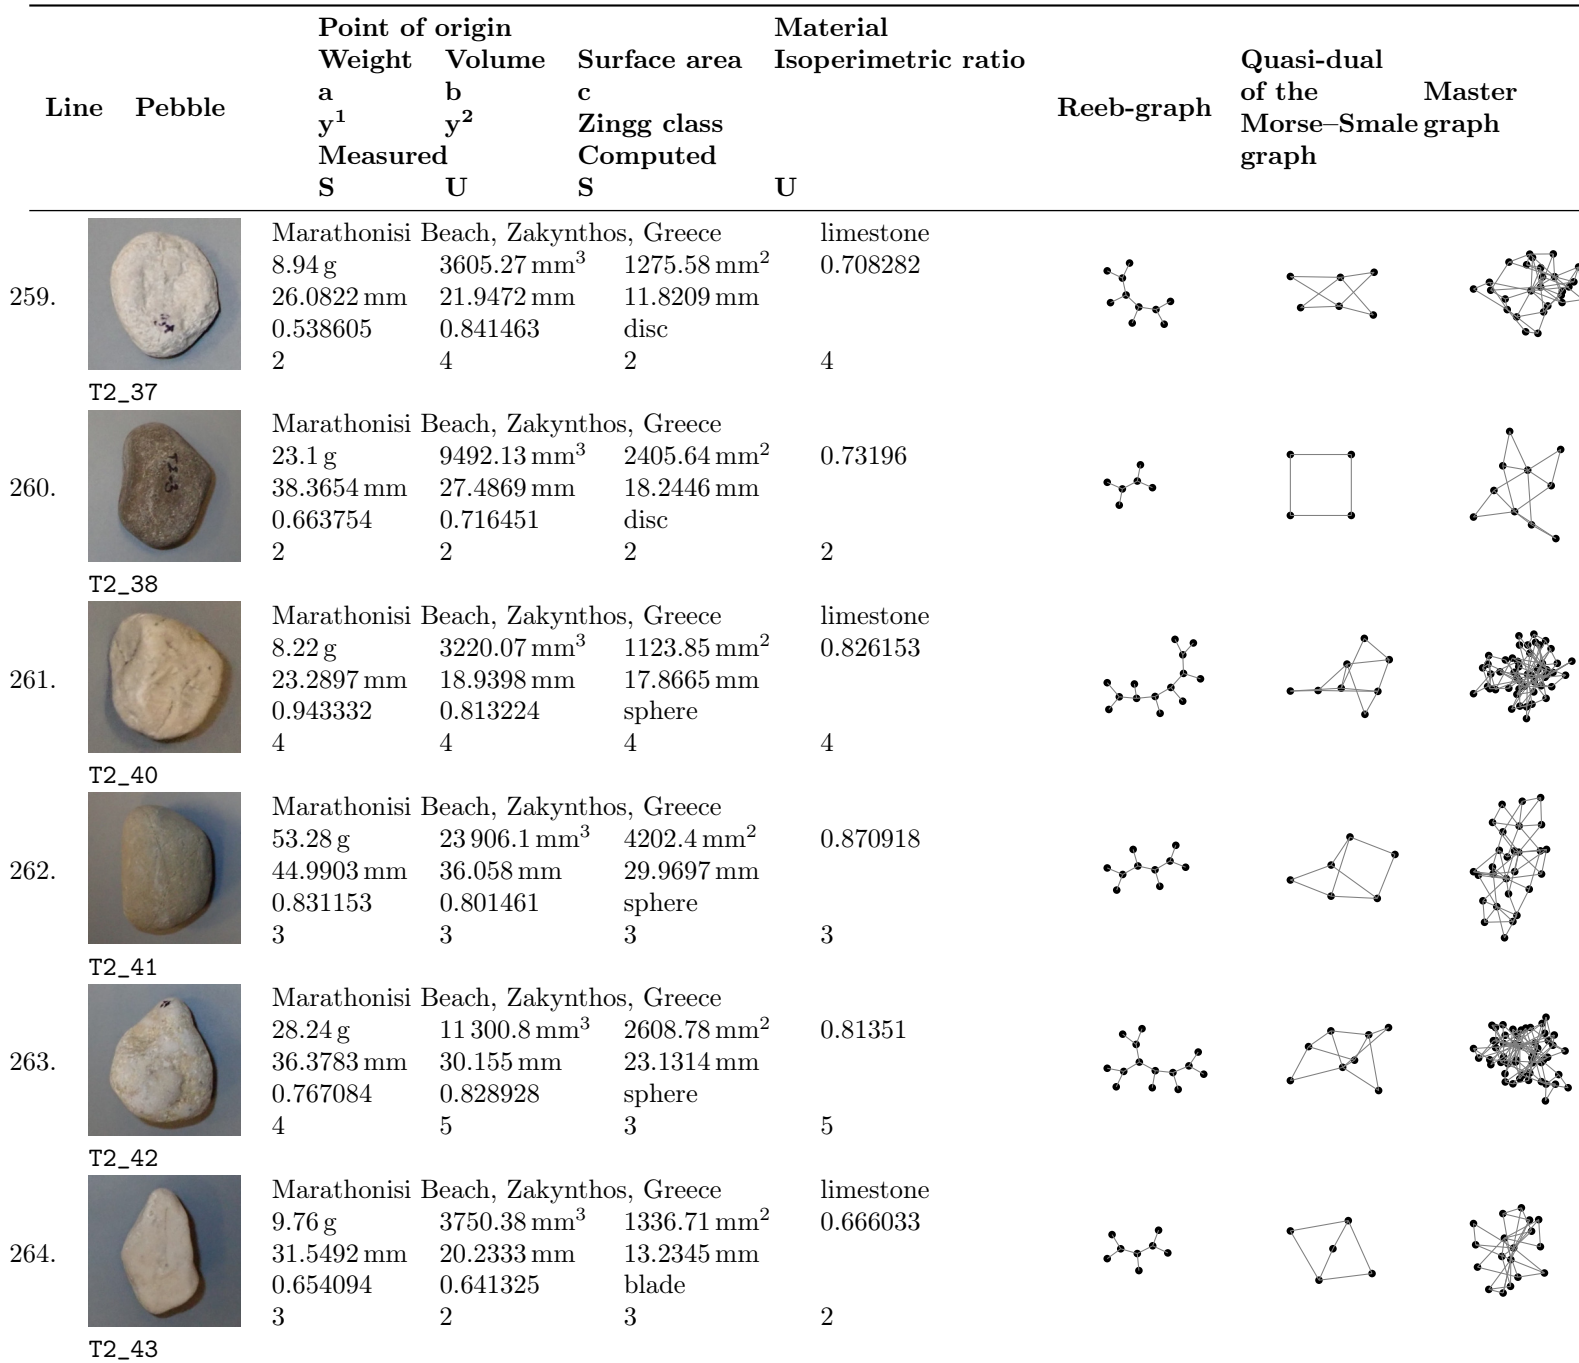 |
|      | T2_43                                                                               |                                                                                |                                                        |                                                      |                                |                     |                                                                                       |                                                                                       |                                                                                       |

| Line | Pebble                                                                              | Point of origin                                                                |                                                                   | Surface area<br>c<br>Zingg class<br>Computed<br>S    | Material<br>Isoperimetric ratio<br>U | Reeb-graph                                                                            | Quasi-dual<br>of the<br>Morse–Smale<br>graph                                          | Master<br>graph                                                                       |
|------|-------------------------------------------------------------------------------------|--------------------------------------------------------------------------------|-------------------------------------------------------------------|------------------------------------------------------|--------------------------------------|---------------------------------------------------------------------------------------|---------------------------------------------------------------------------------------|---------------------------------------------------------------------------------------|
|      |                                                                                     | Weight                                                                         | Volume                                                            |                                                      |                                      |                                                                                       |                                                                                       |                                                                                       |
|      |                                                                                     | a<br>y <sup>1</sup><br>Measured<br>S                                           | b<br>y <sup>2</sup><br>U                                          |                                                      |                                      |                                                                                       |                                                                                       |                                                                                       |
|      |                                                                                     |                                                                                |                                                                   |                                                      |                                      |                                                                                       |                                                                                       |                                                                                       |
| 265. | 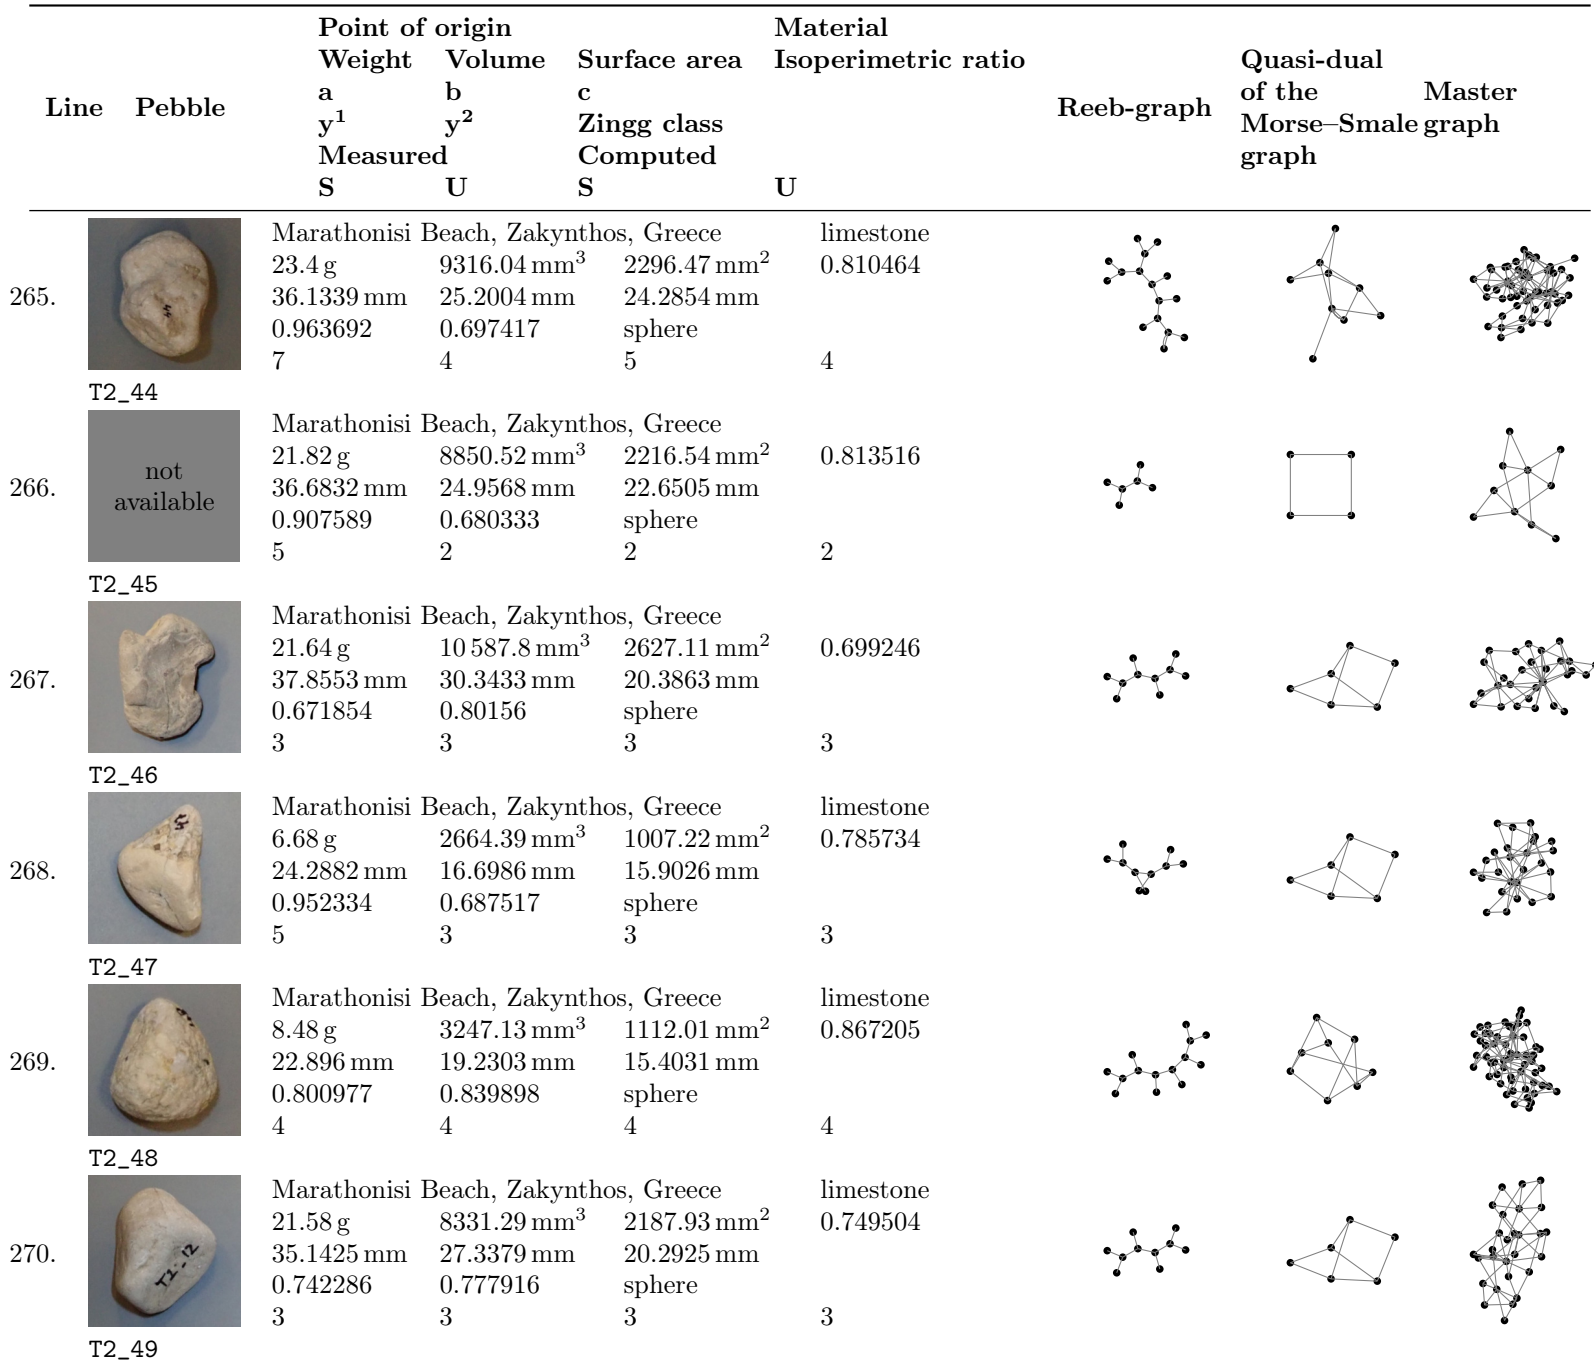   | Marathonisi Beach, Zakynthos, Greece<br>23.4 g<br>36.1339 mm<br>0.963692<br>7  | 23.4 g<br>9316.04 mm <sup>3</sup><br>25.2004 mm<br>0.697417<br>4  | 2296.47 mm <sup>2</sup><br>24.2854 mm<br>sphere<br>5 | limestone<br>0.810464<br><br>4       | 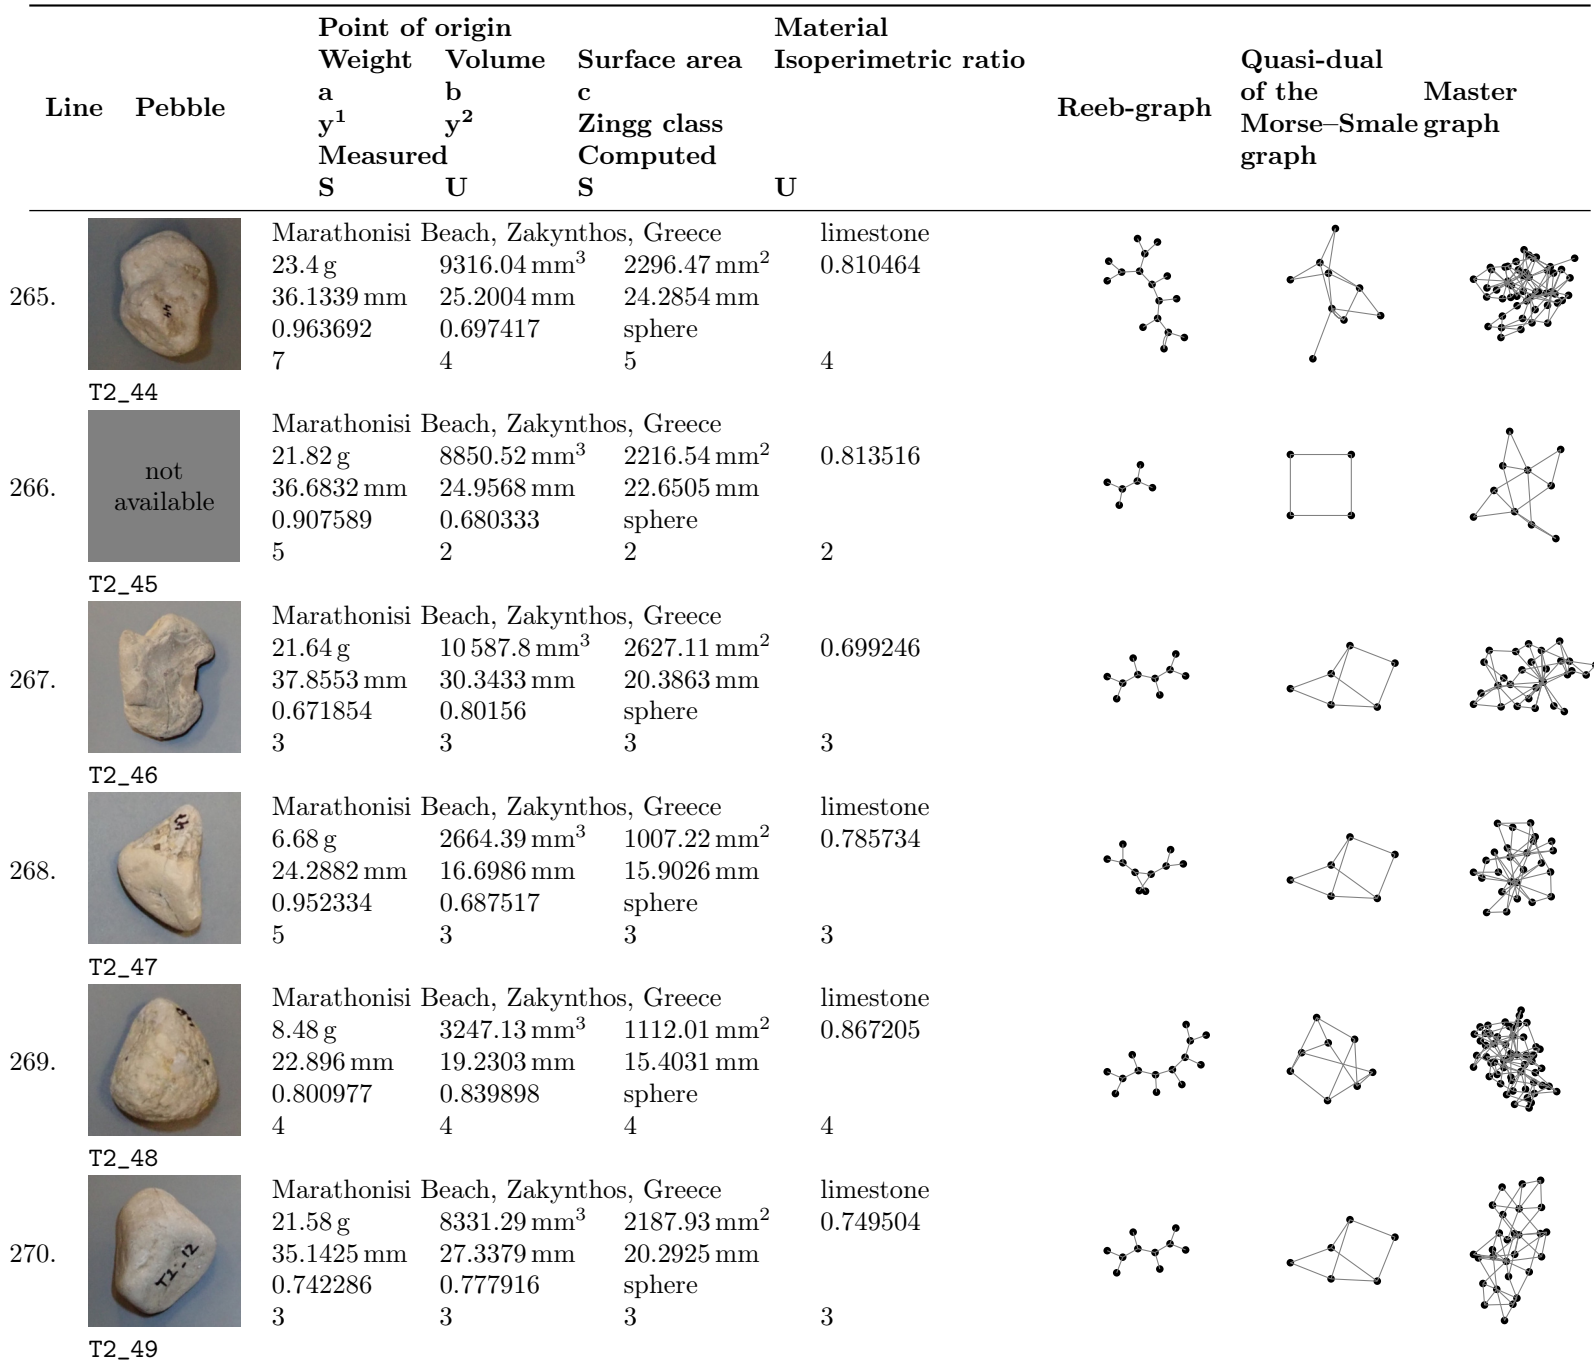   | 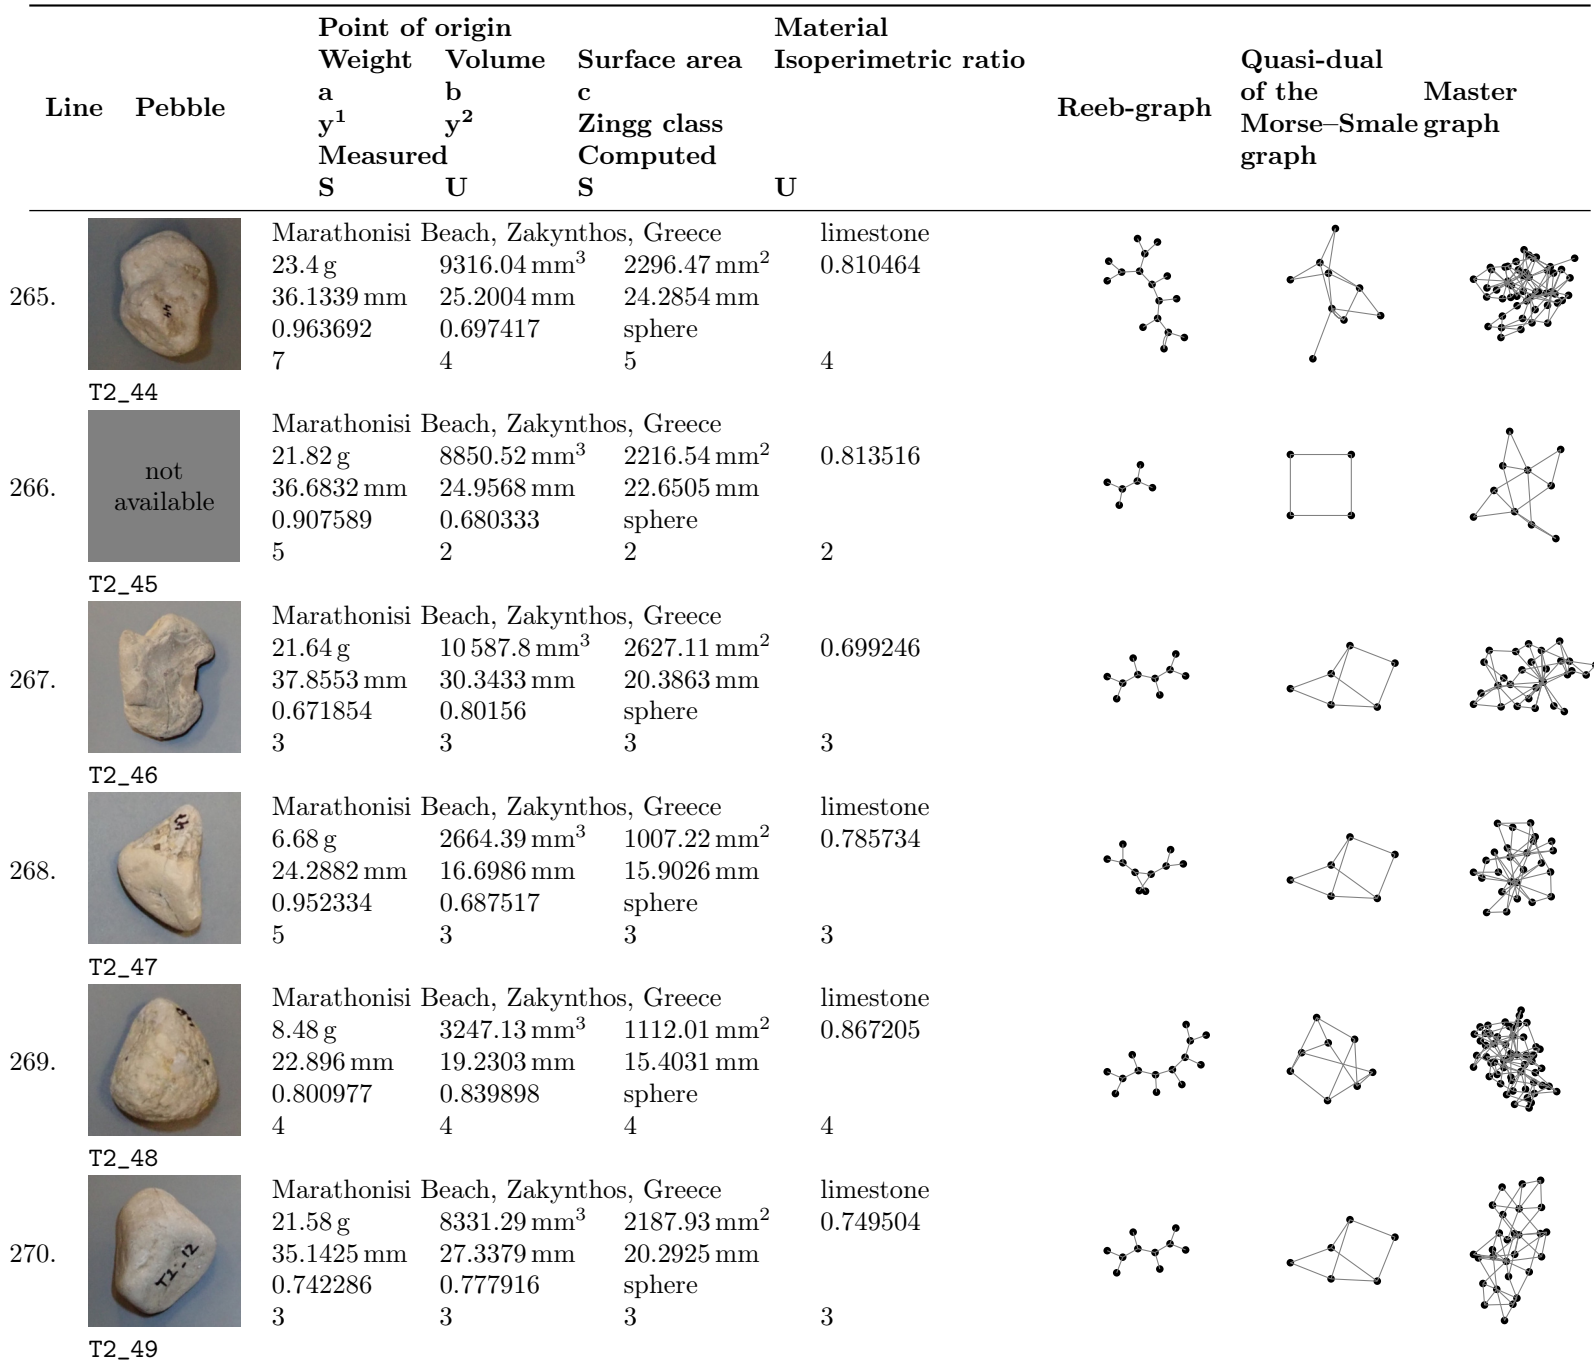   | 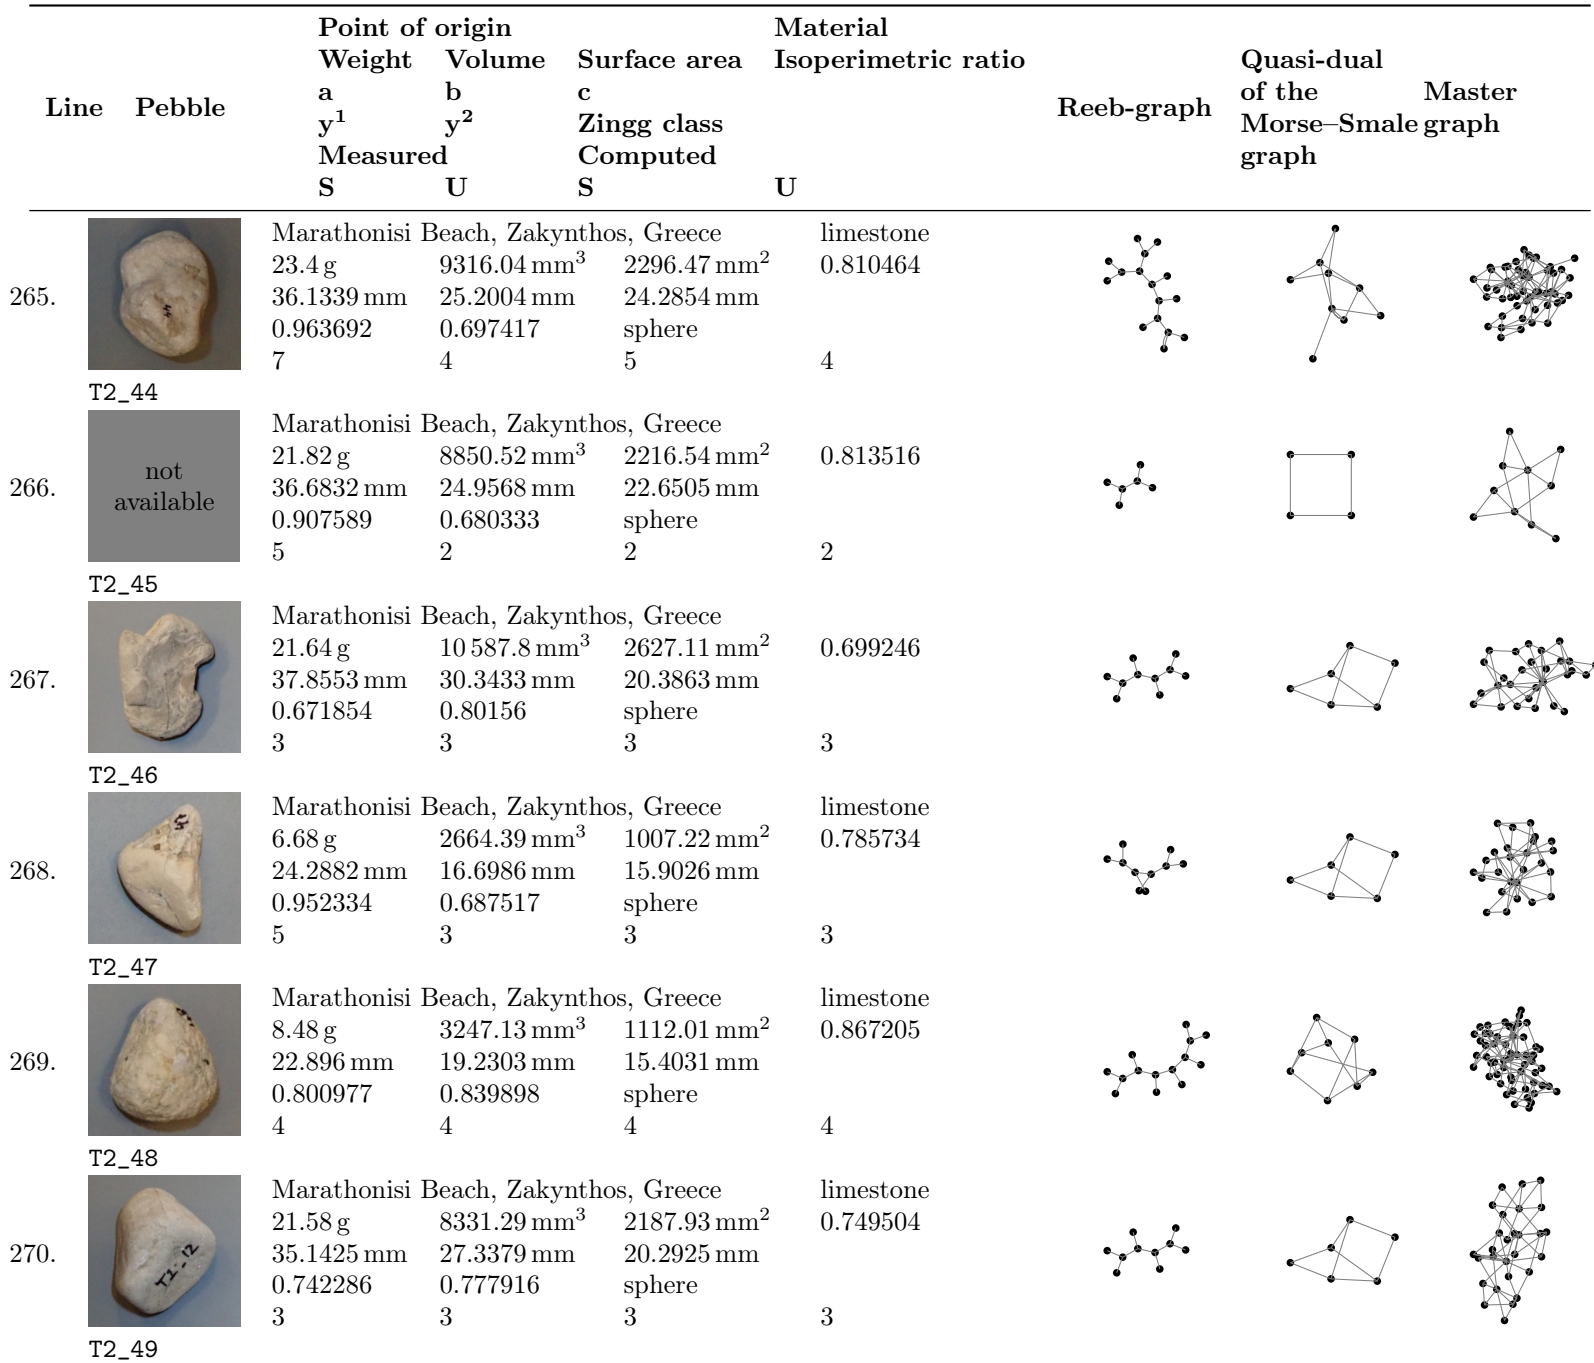   |
|      | T2_44                                                                               |                                                                                |                                                                   |                                                      |                                      |                                                                                       |                                                                                       |                                                                                       |
| 266. | 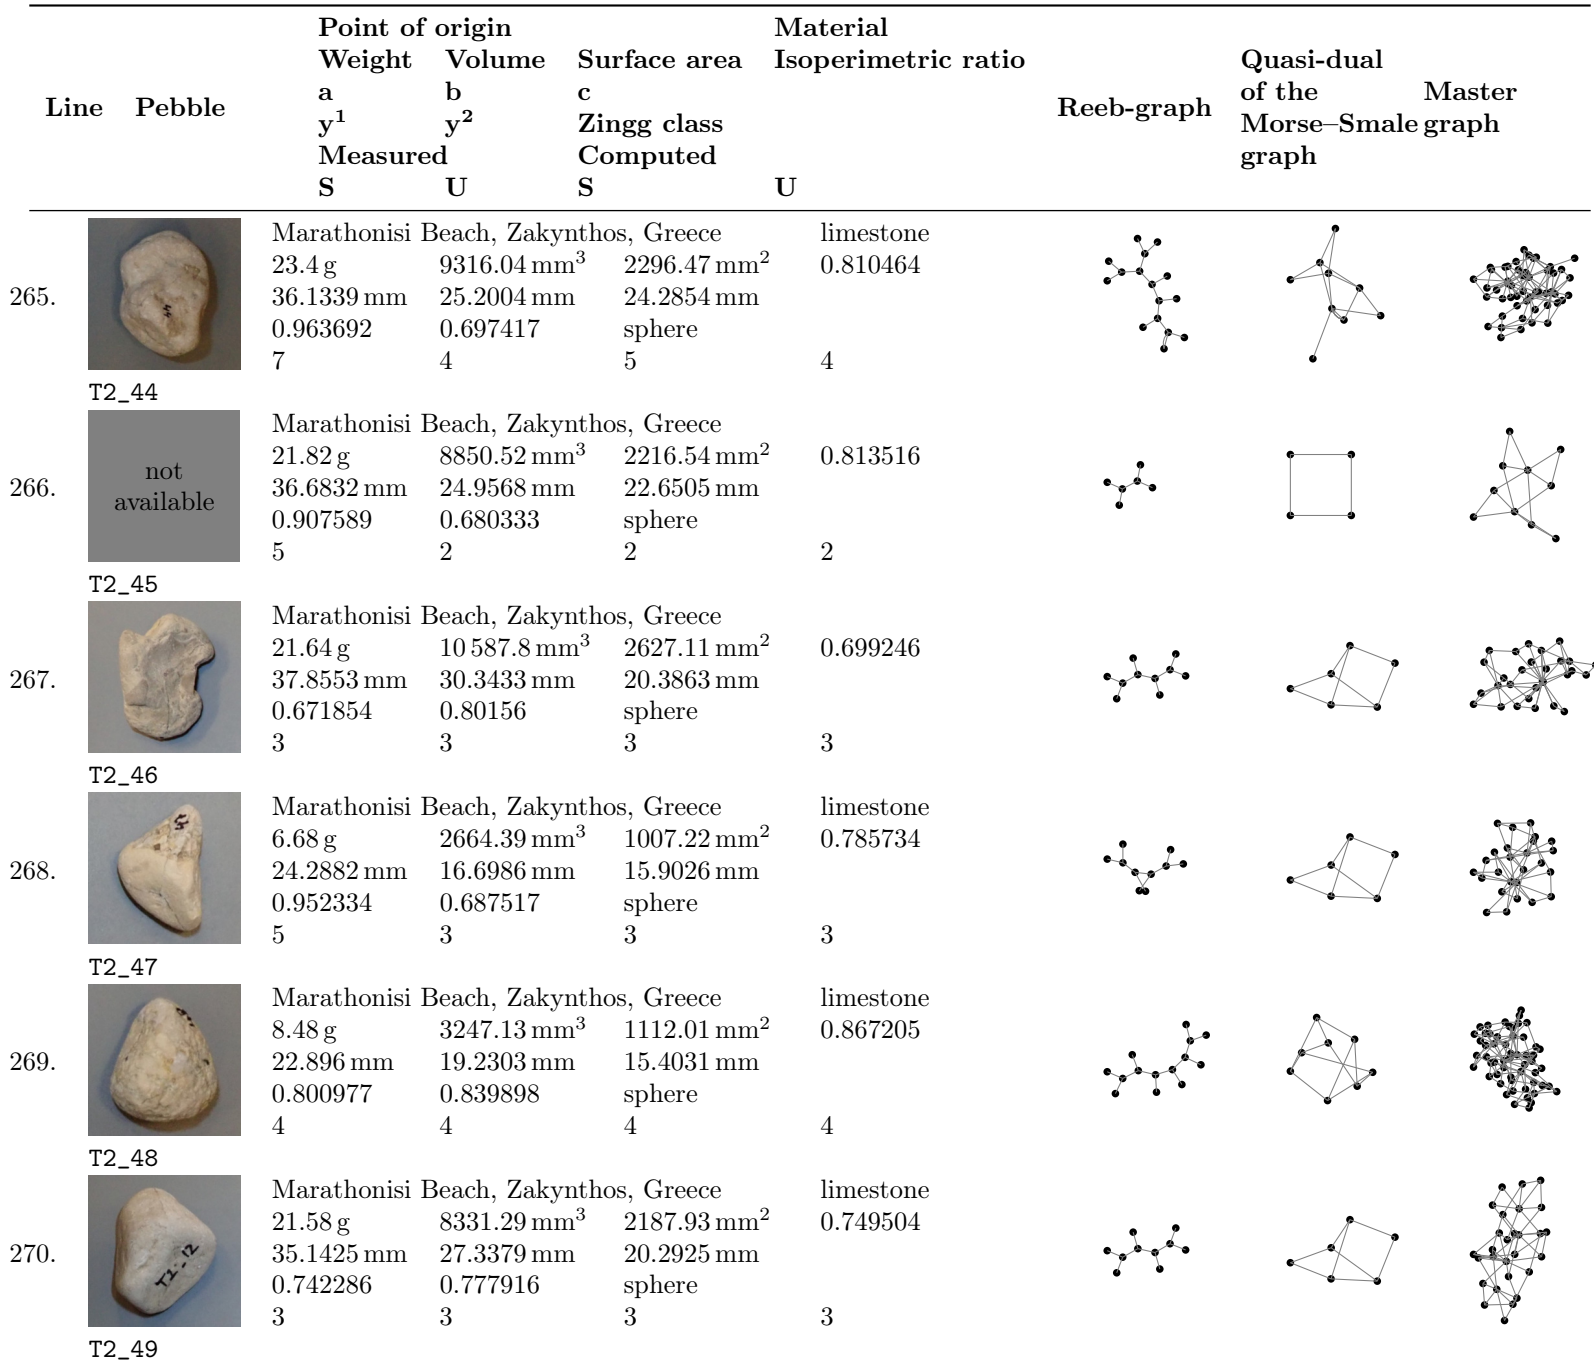   | Marathonisi Beach, Zakynthos, Greece<br>21.82 g<br>36.6832 mm<br>0.907589<br>5 | 21.82 g<br>8850.52 mm <sup>3</sup><br>24.9568 mm<br>0.680333<br>2 | 2216.54 mm <sup>2</sup><br>22.6505 mm<br>sphere<br>2 | 0.813516<br><br>2                    | 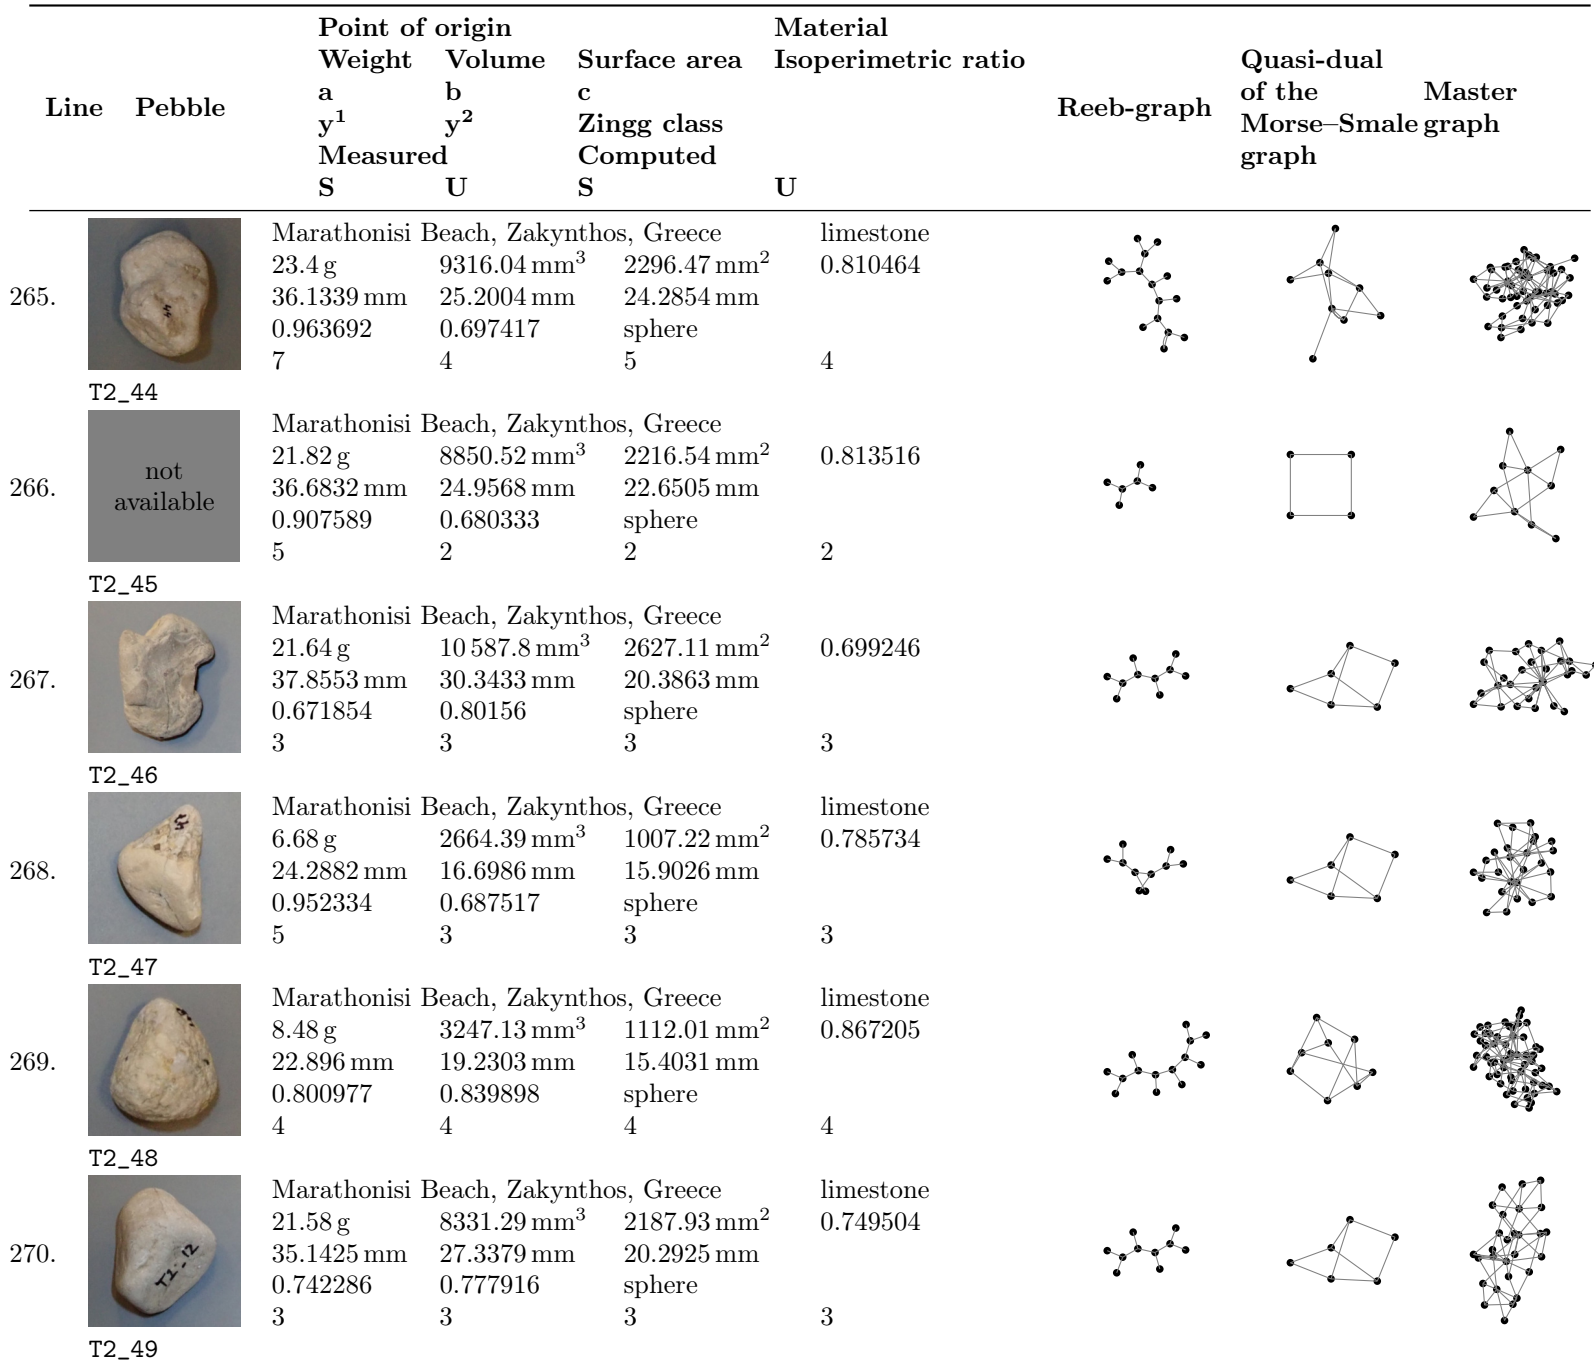   | 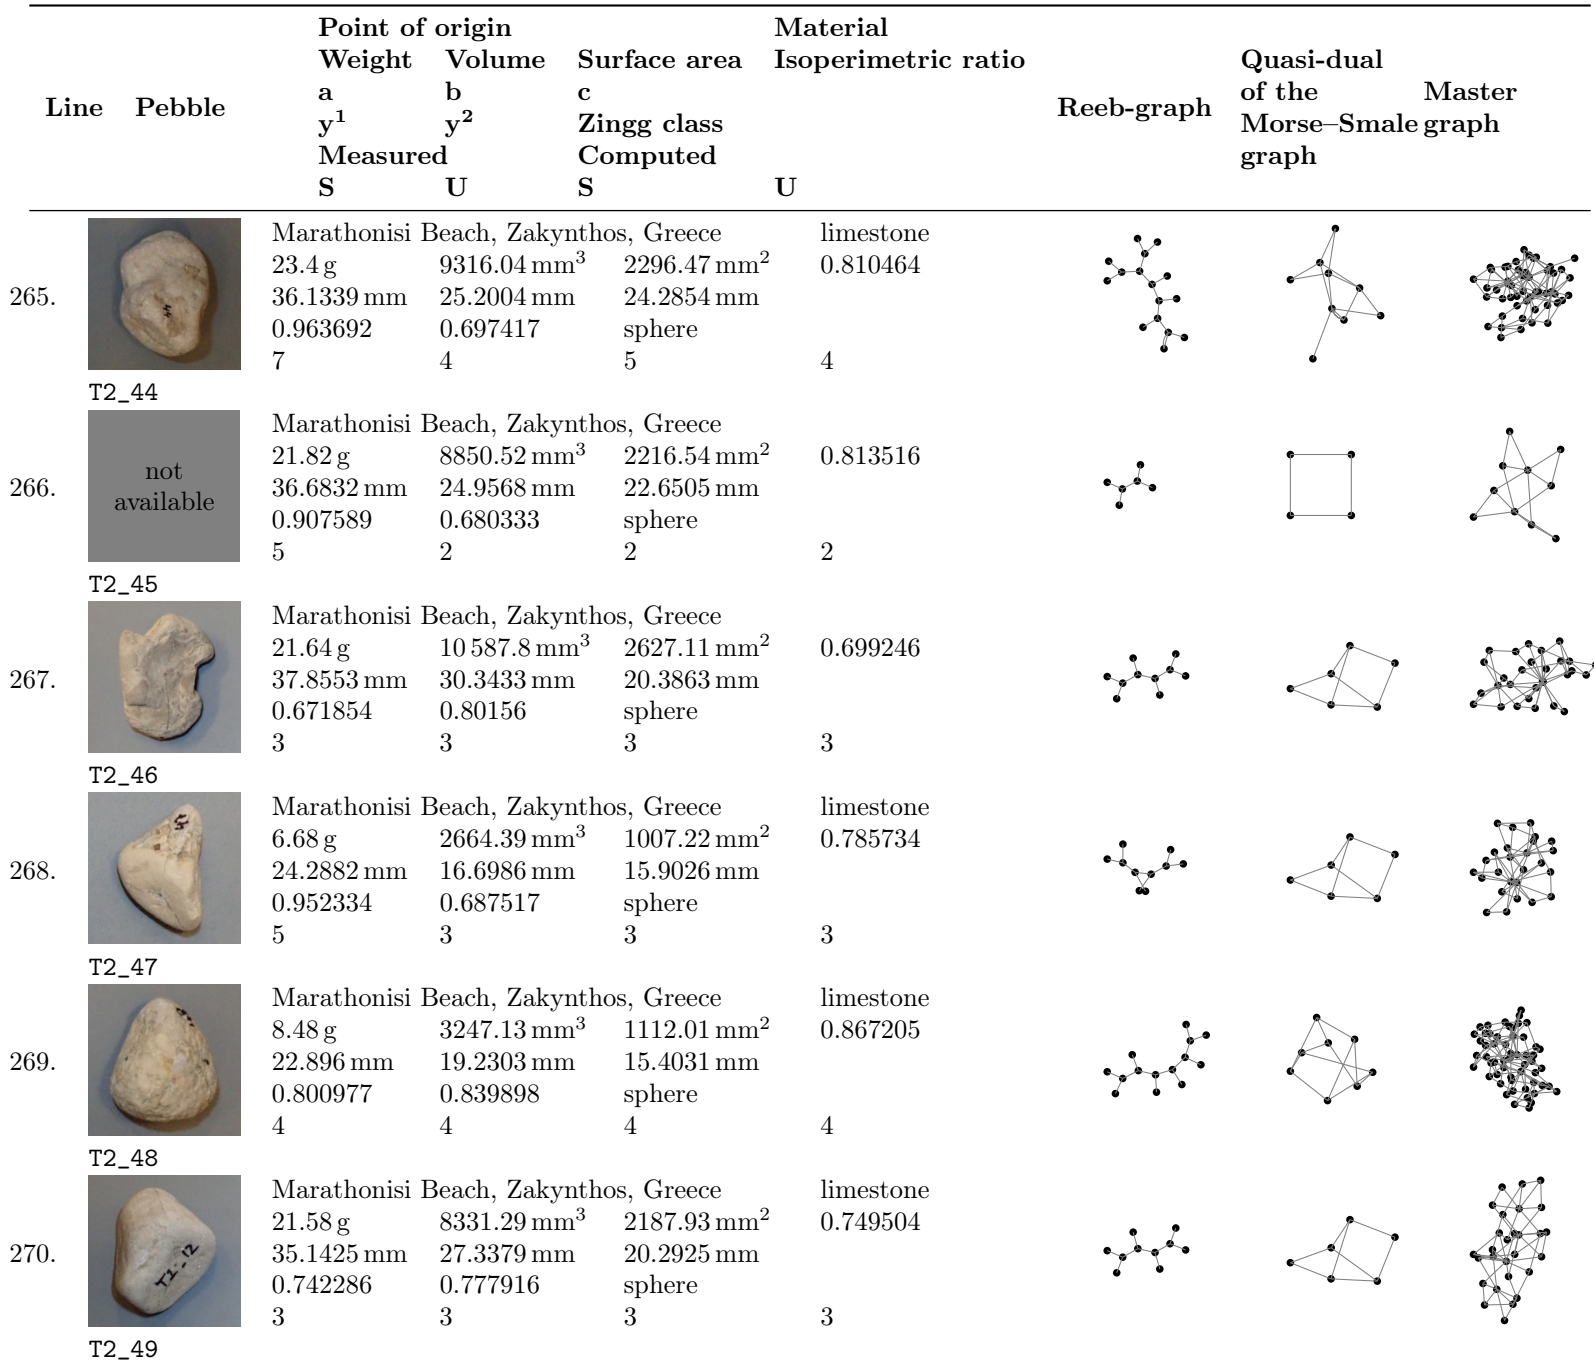   | 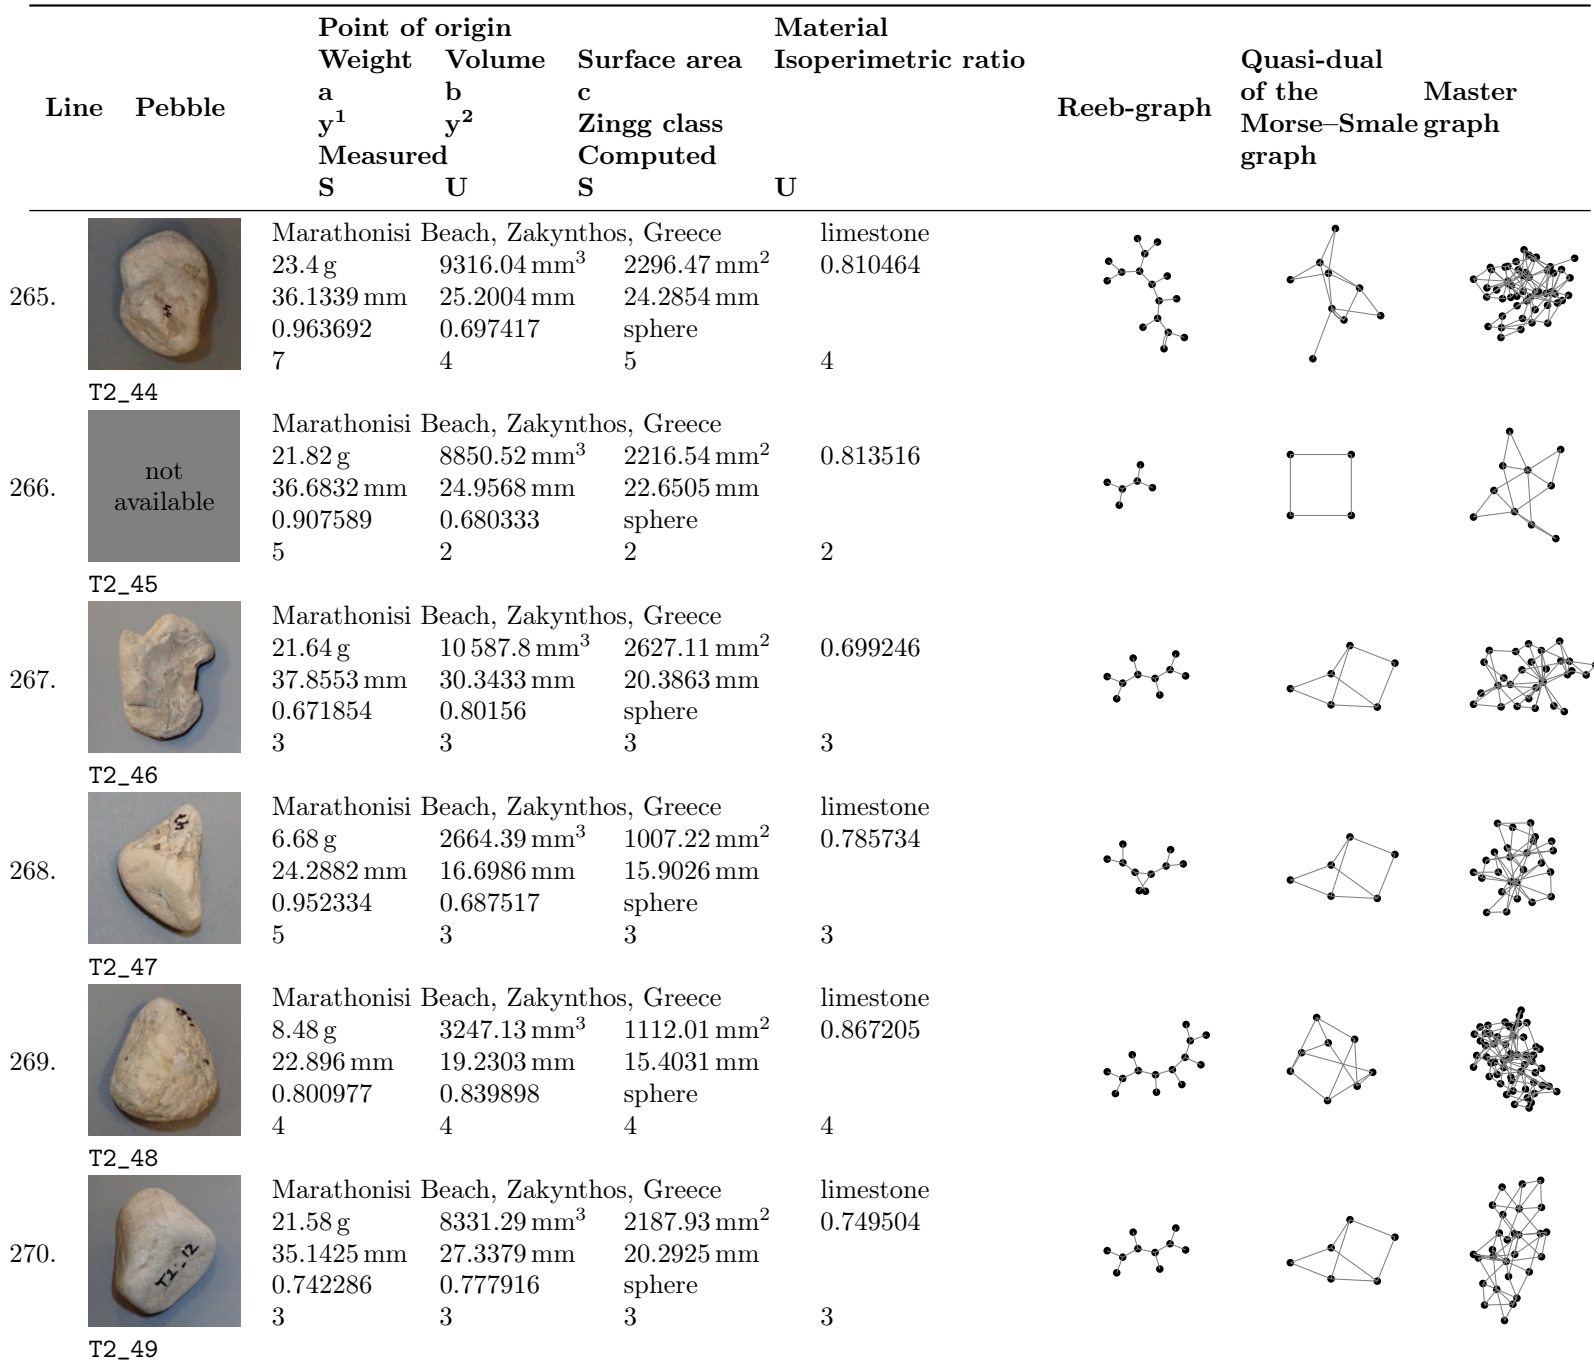   |
|      | T2_45                                                                               |                                                                                |                                                                   |                                                      |                                      |                                                                                       |                                                                                       |                                                                                       |
| 267. | 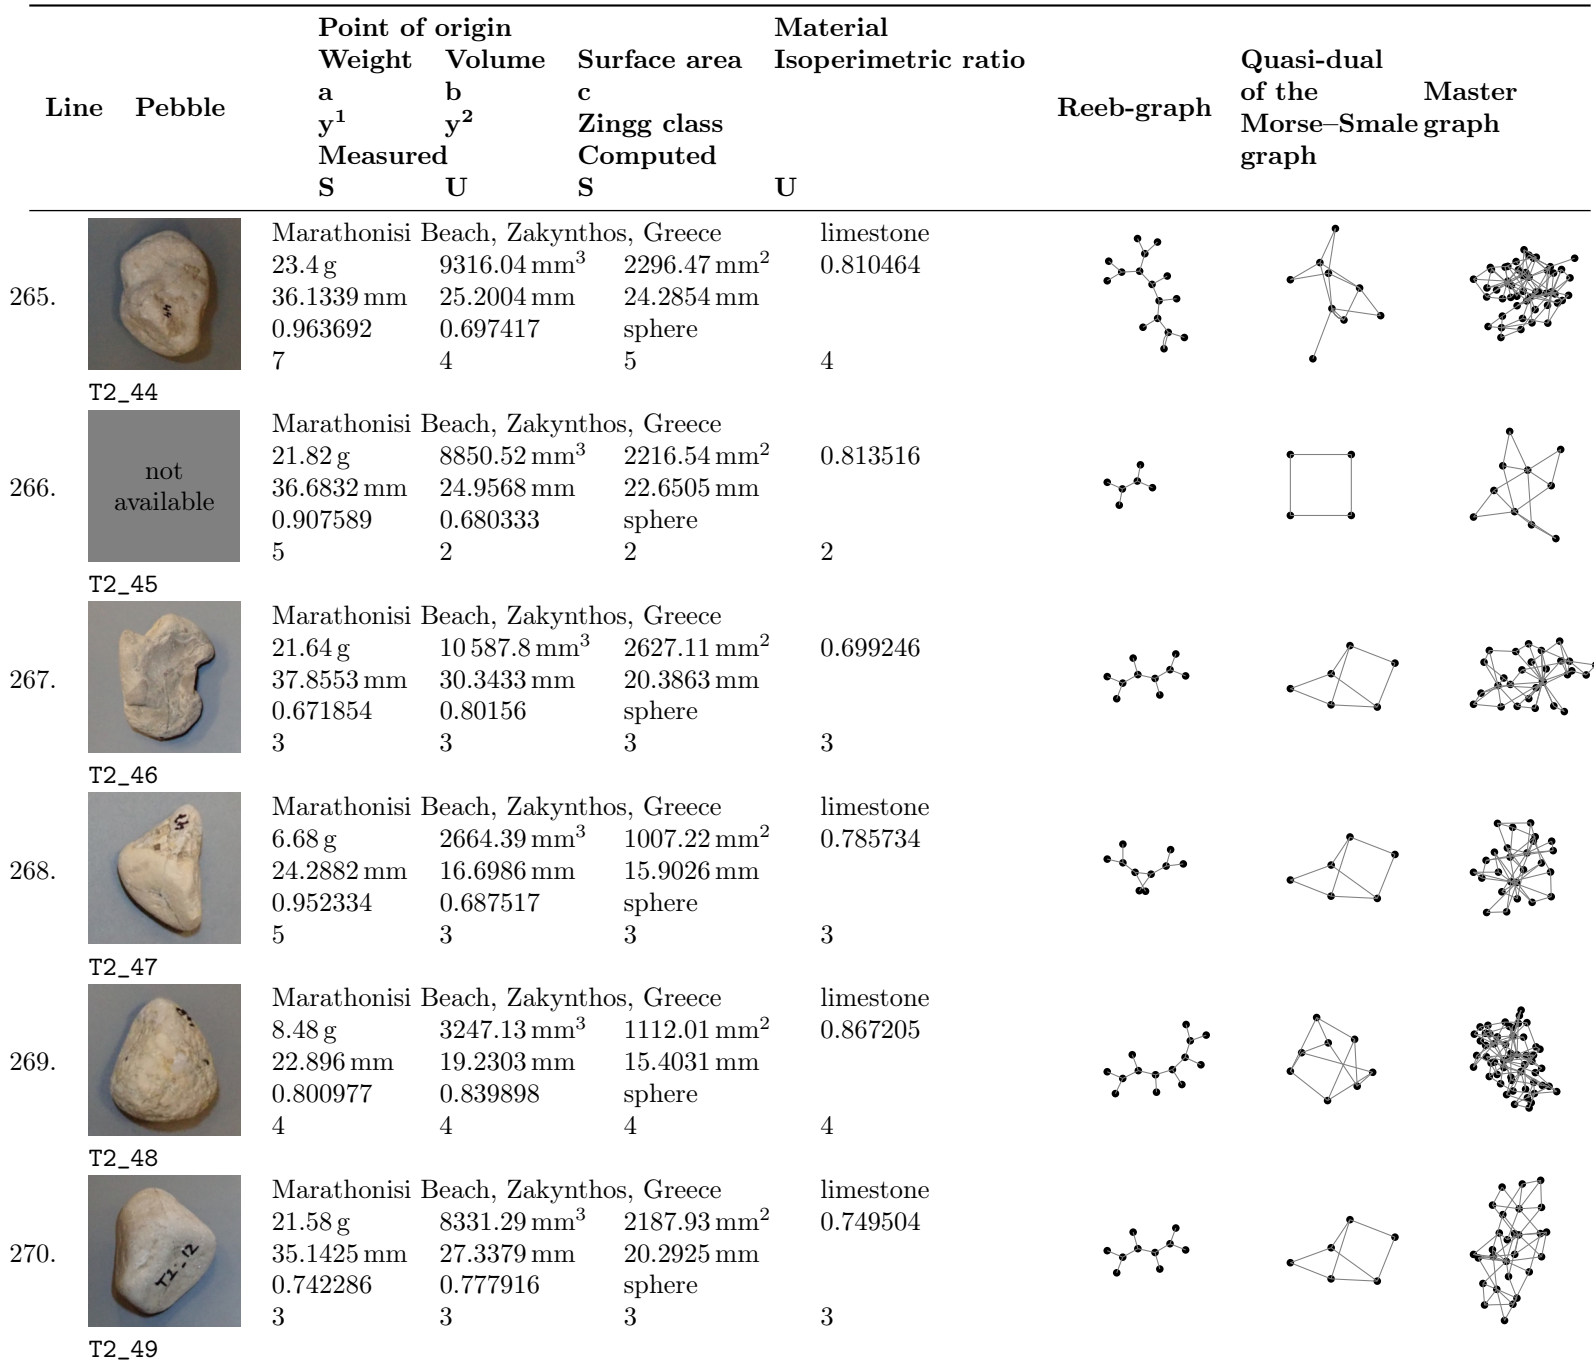   | Marathonisi Beach, Zakynthos, Greece<br>21.64 g<br>37.8553 mm<br>0.671854<br>3 | 21.64 g<br>10 587.8 mm <sup>3</sup><br>30.3433 mm<br>0.80156<br>3 | 2627.11 mm <sup>2</sup><br>20.3863 mm<br>sphere<br>3 | 0.699246<br><br>3                    | 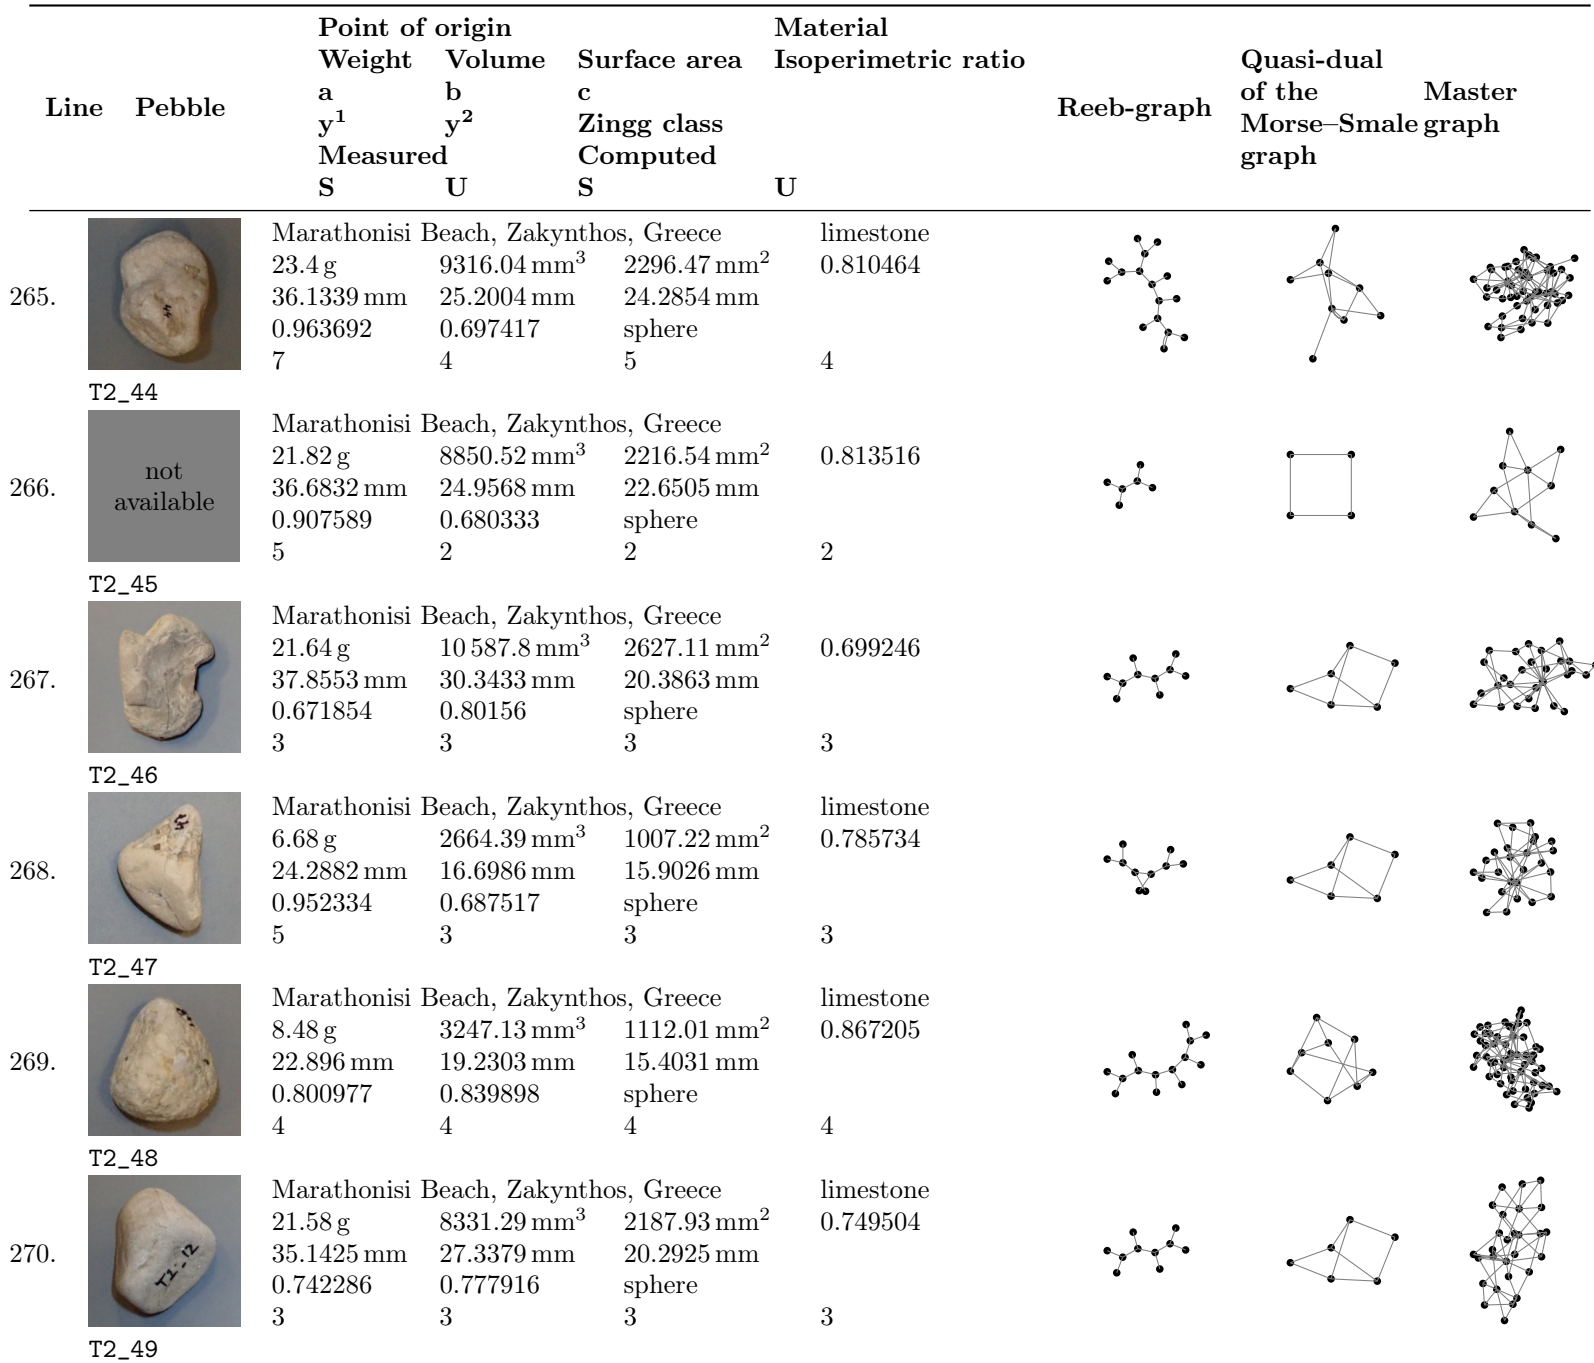   | 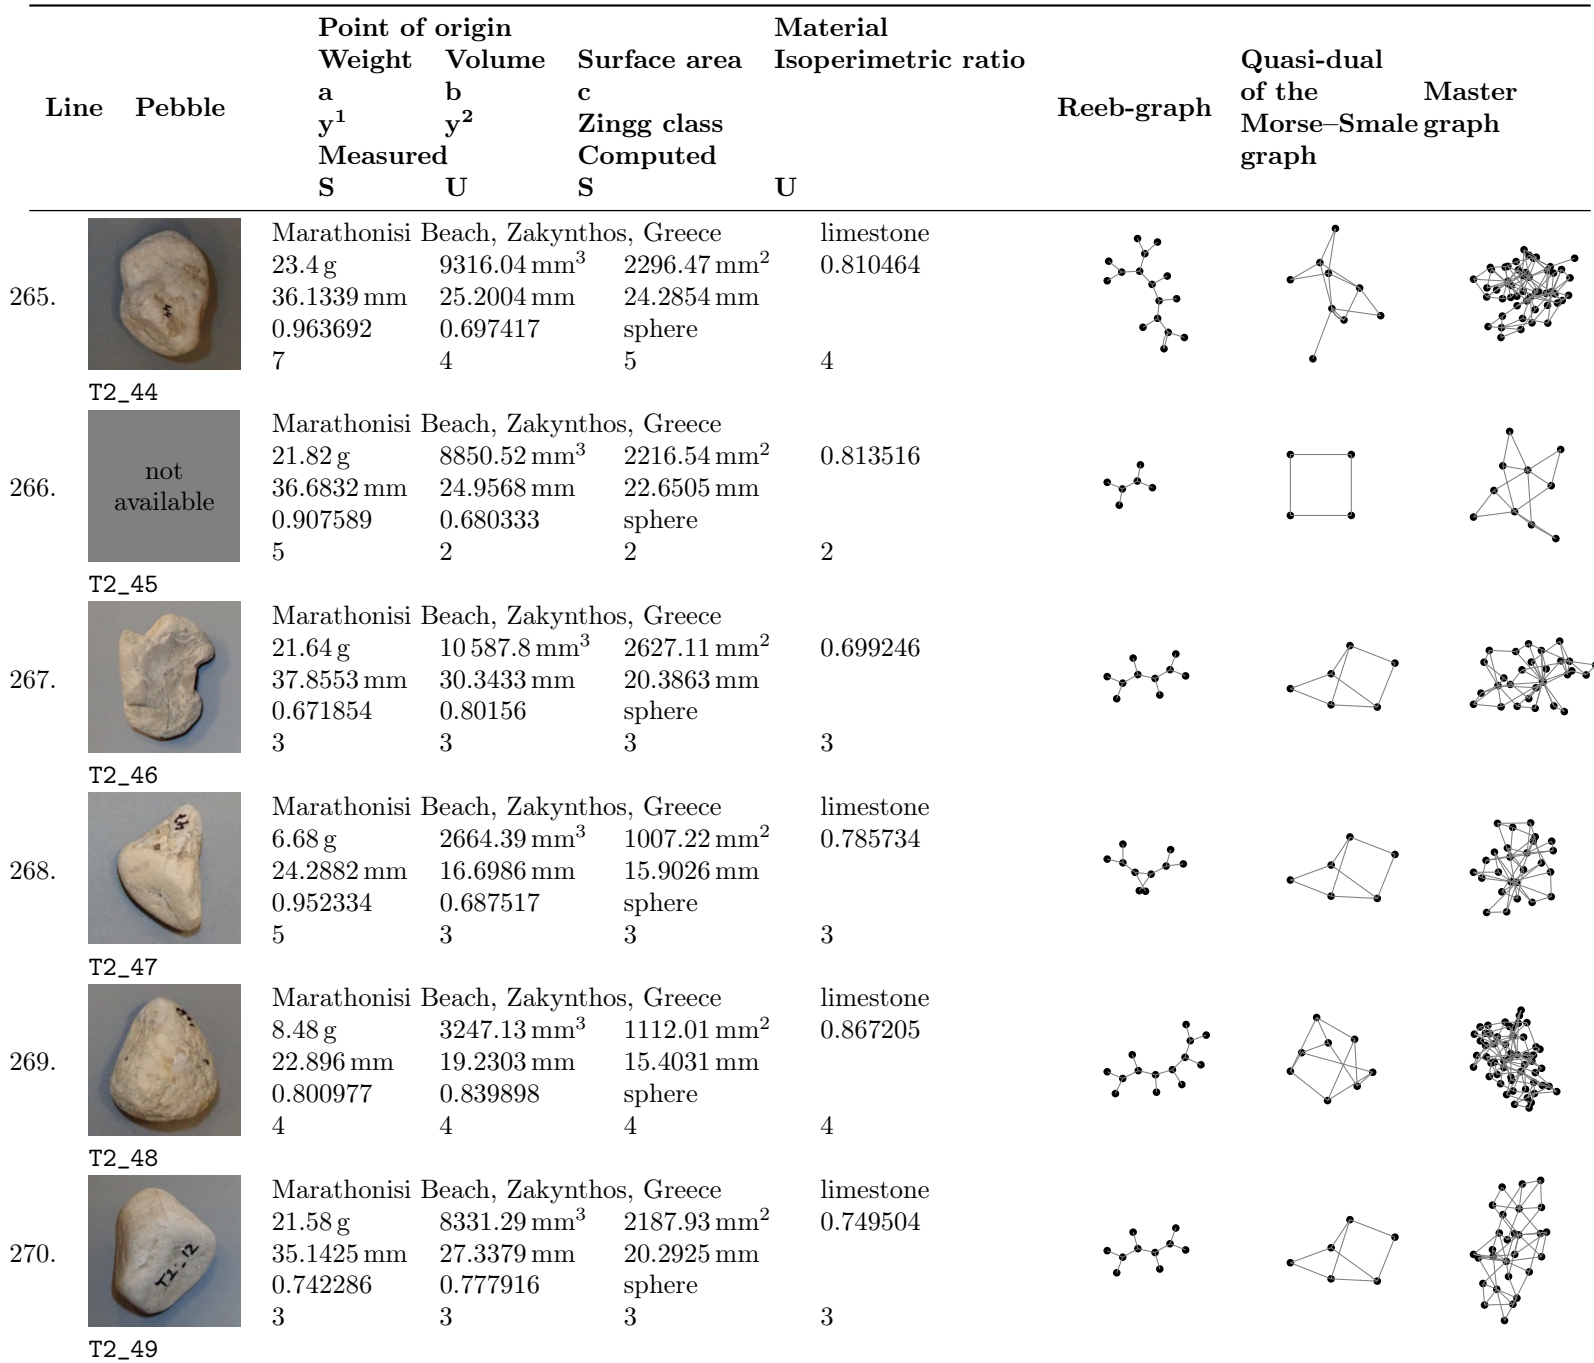   | 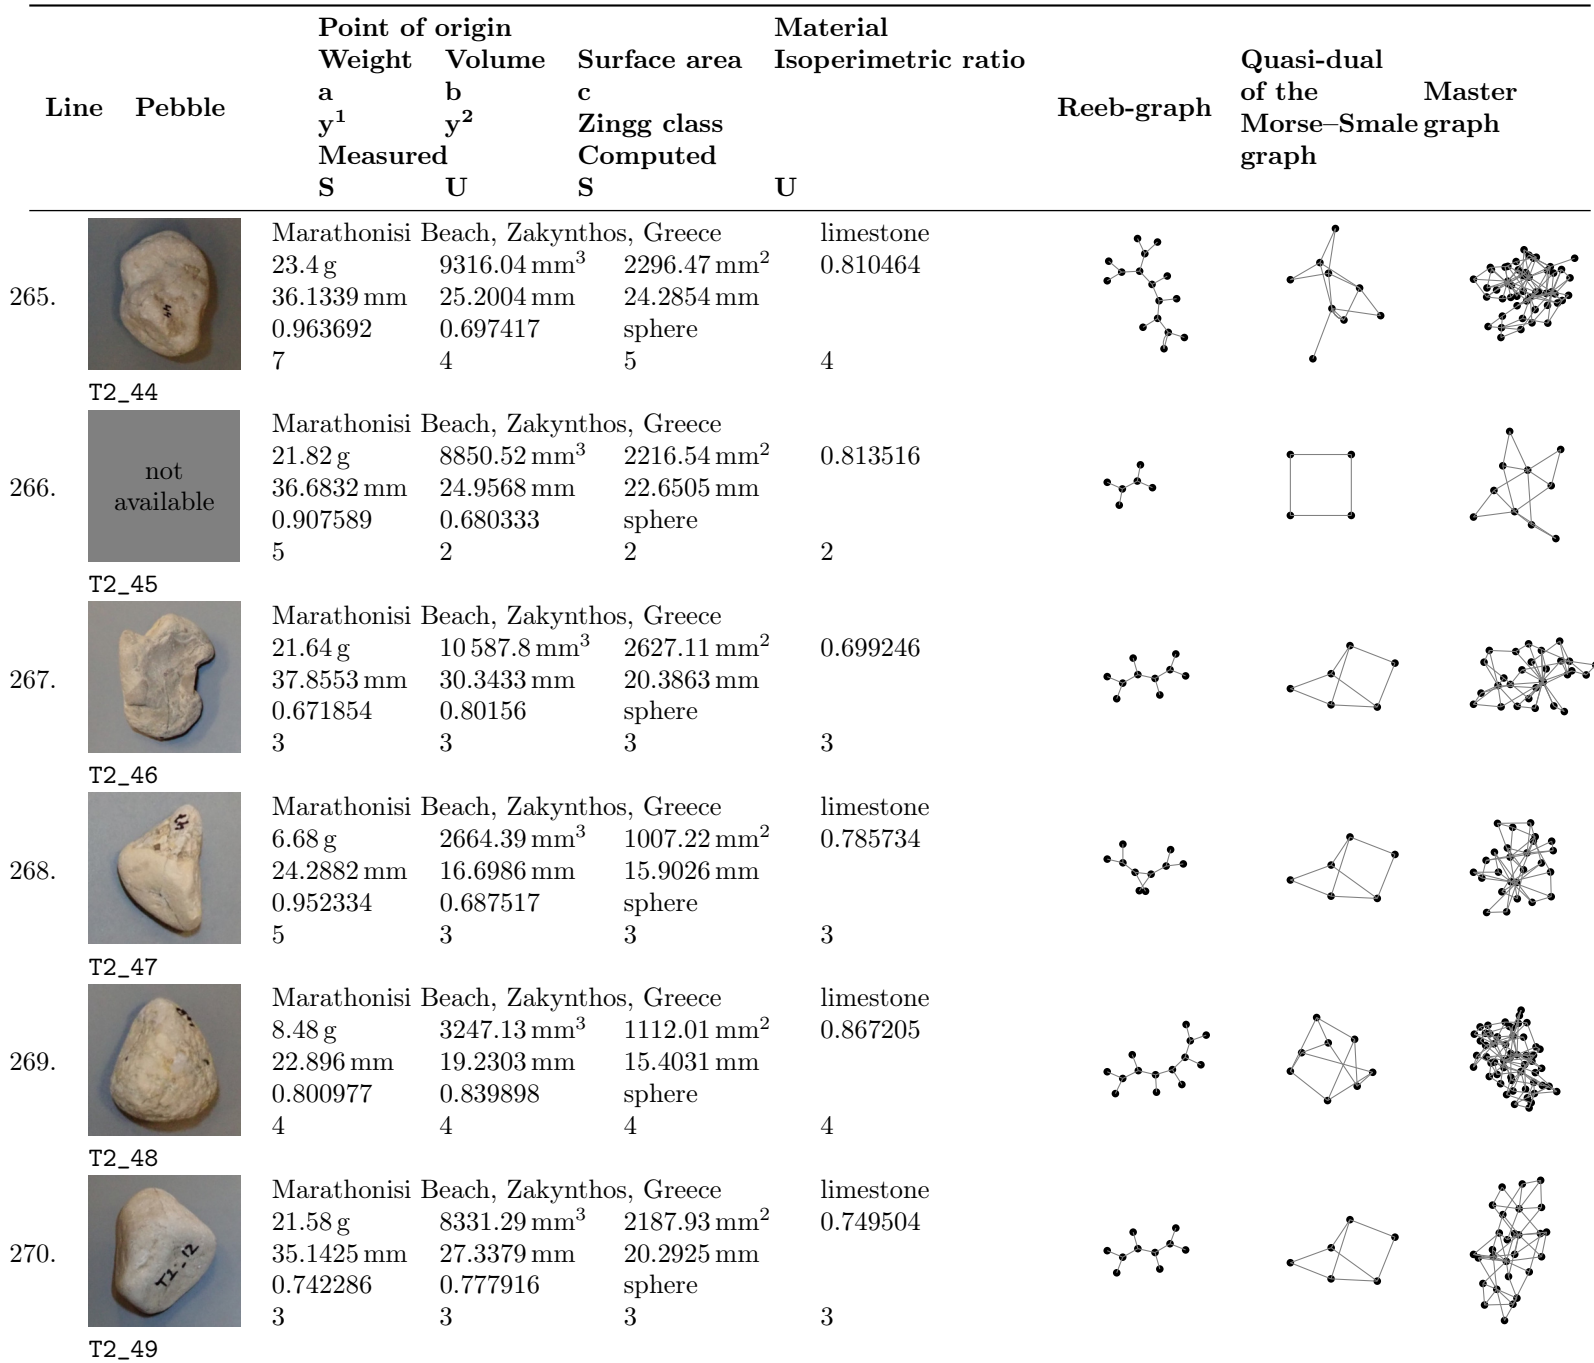   |
|      | T2_46                                                                               |                                                                                |                                                                   |                                                      |                                      |                                                                                       |                                                                                       |                                                                                       |
| 268. | 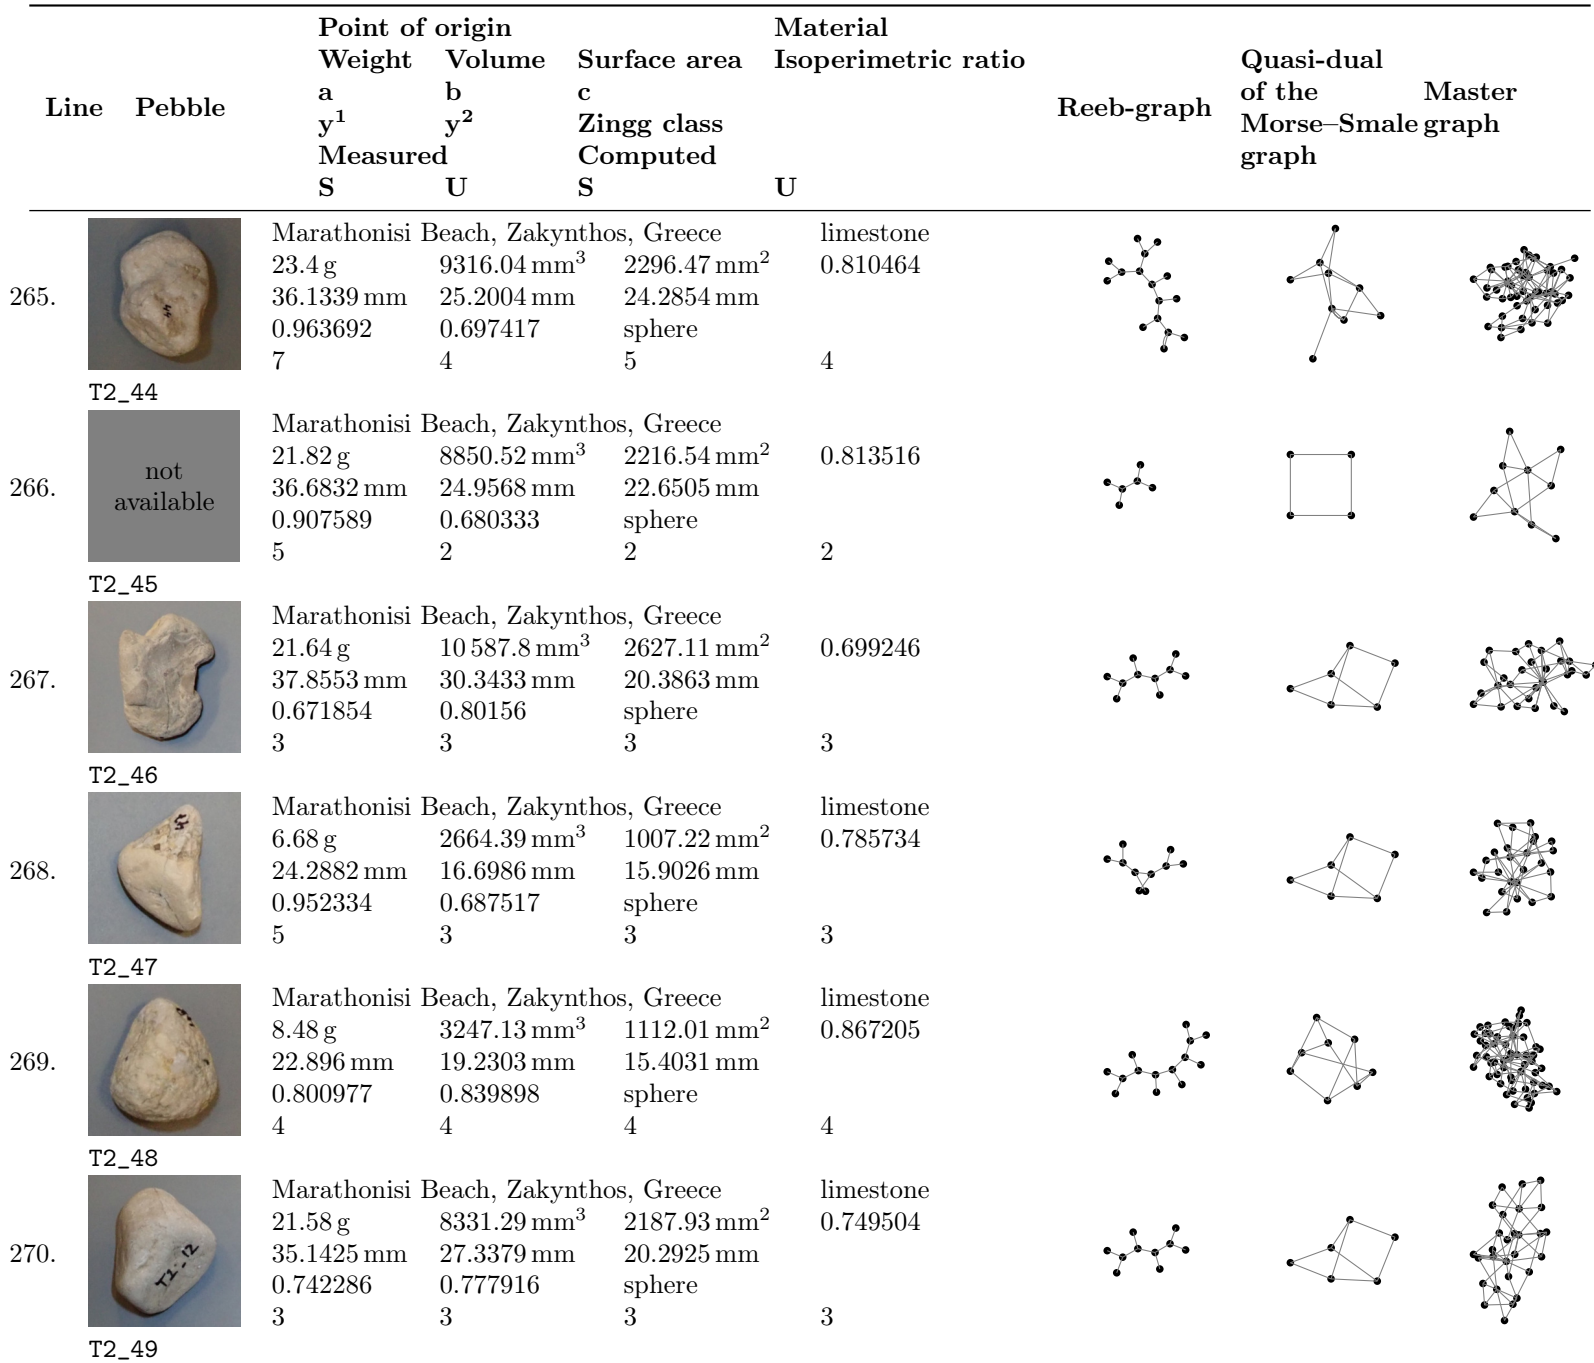  | Marathonisi Beach, Zakynthos, Greece<br>6.68 g<br>24.2882 mm<br>0.952334<br>5  | 6.68 g<br>2664.39 mm <sup>3</sup><br>16.6986 mm<br>0.687517<br>3  | 1007.22 mm <sup>2</sup><br>15.9026 mm<br>sphere<br>3 | limestone<br>0.785734<br><br>3       | 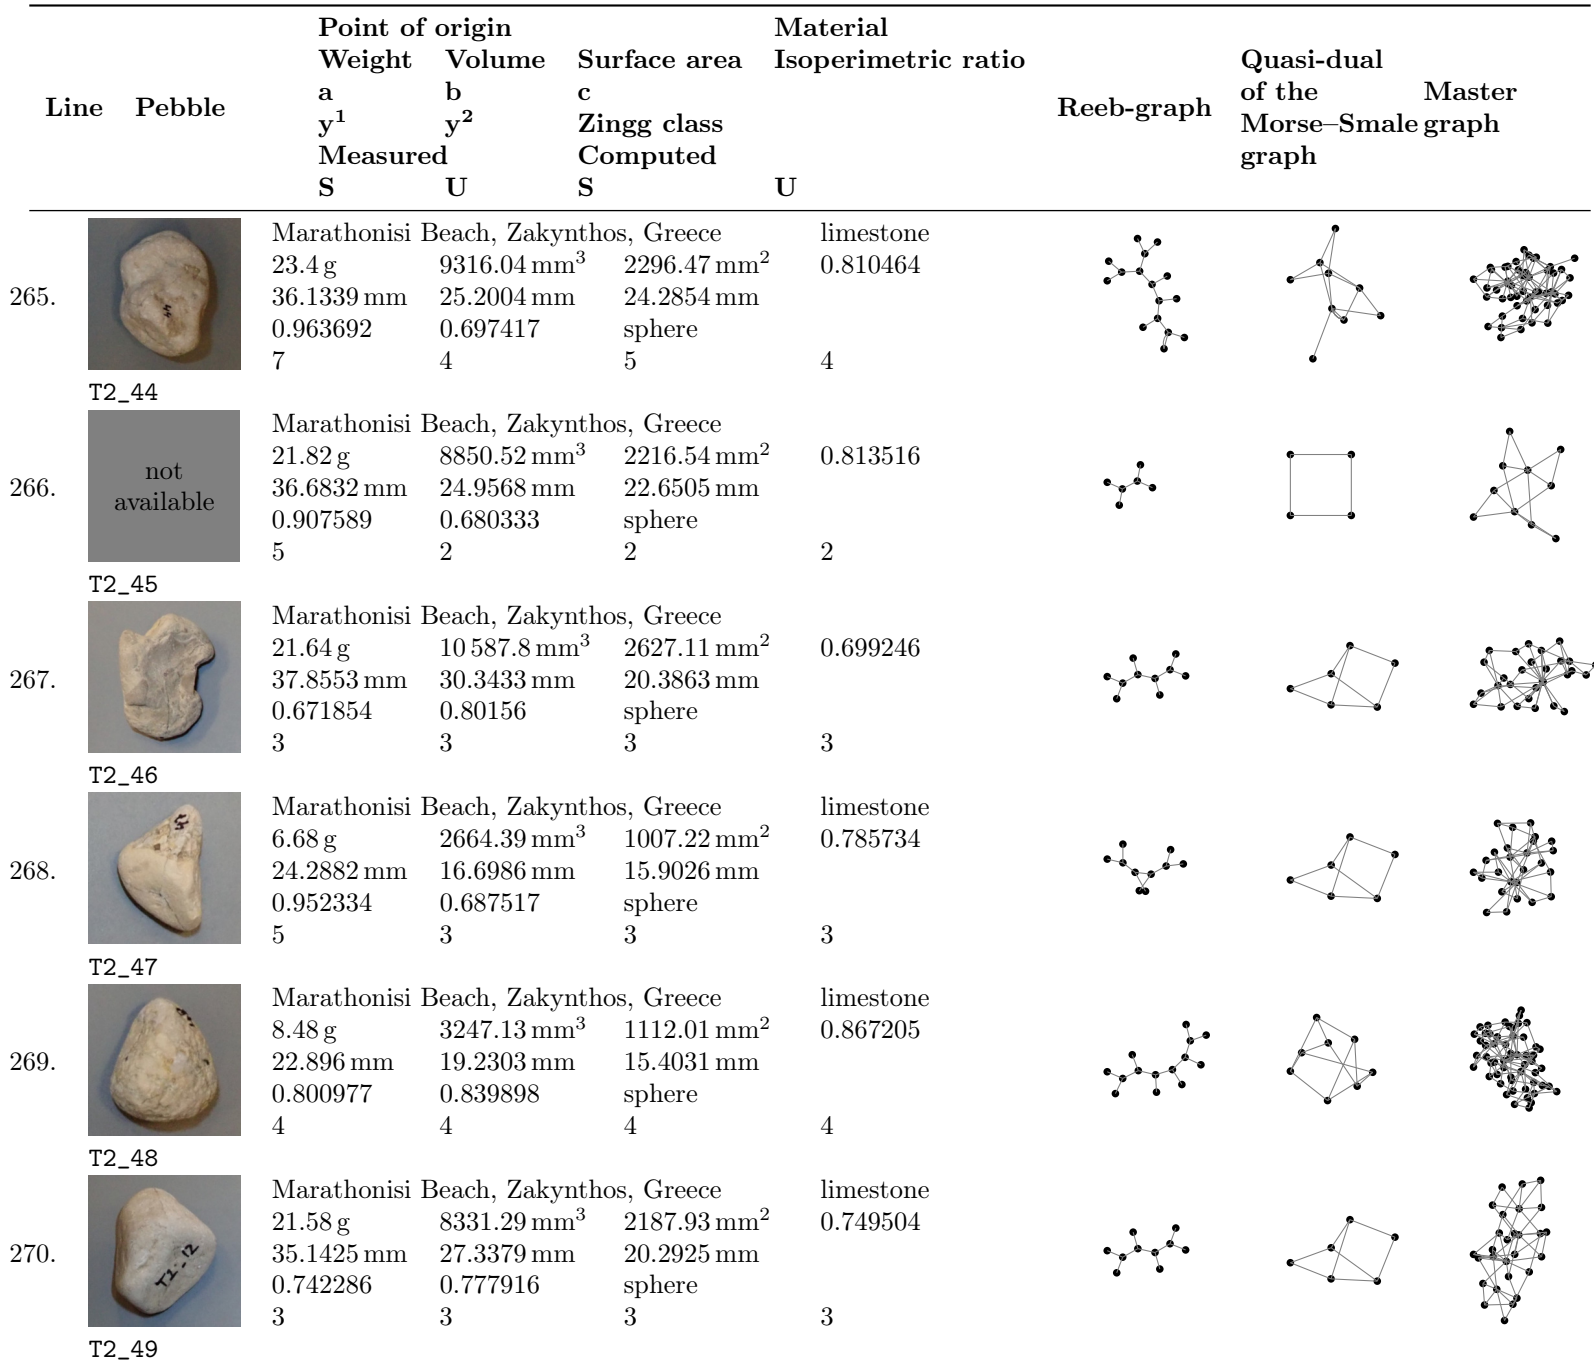  | 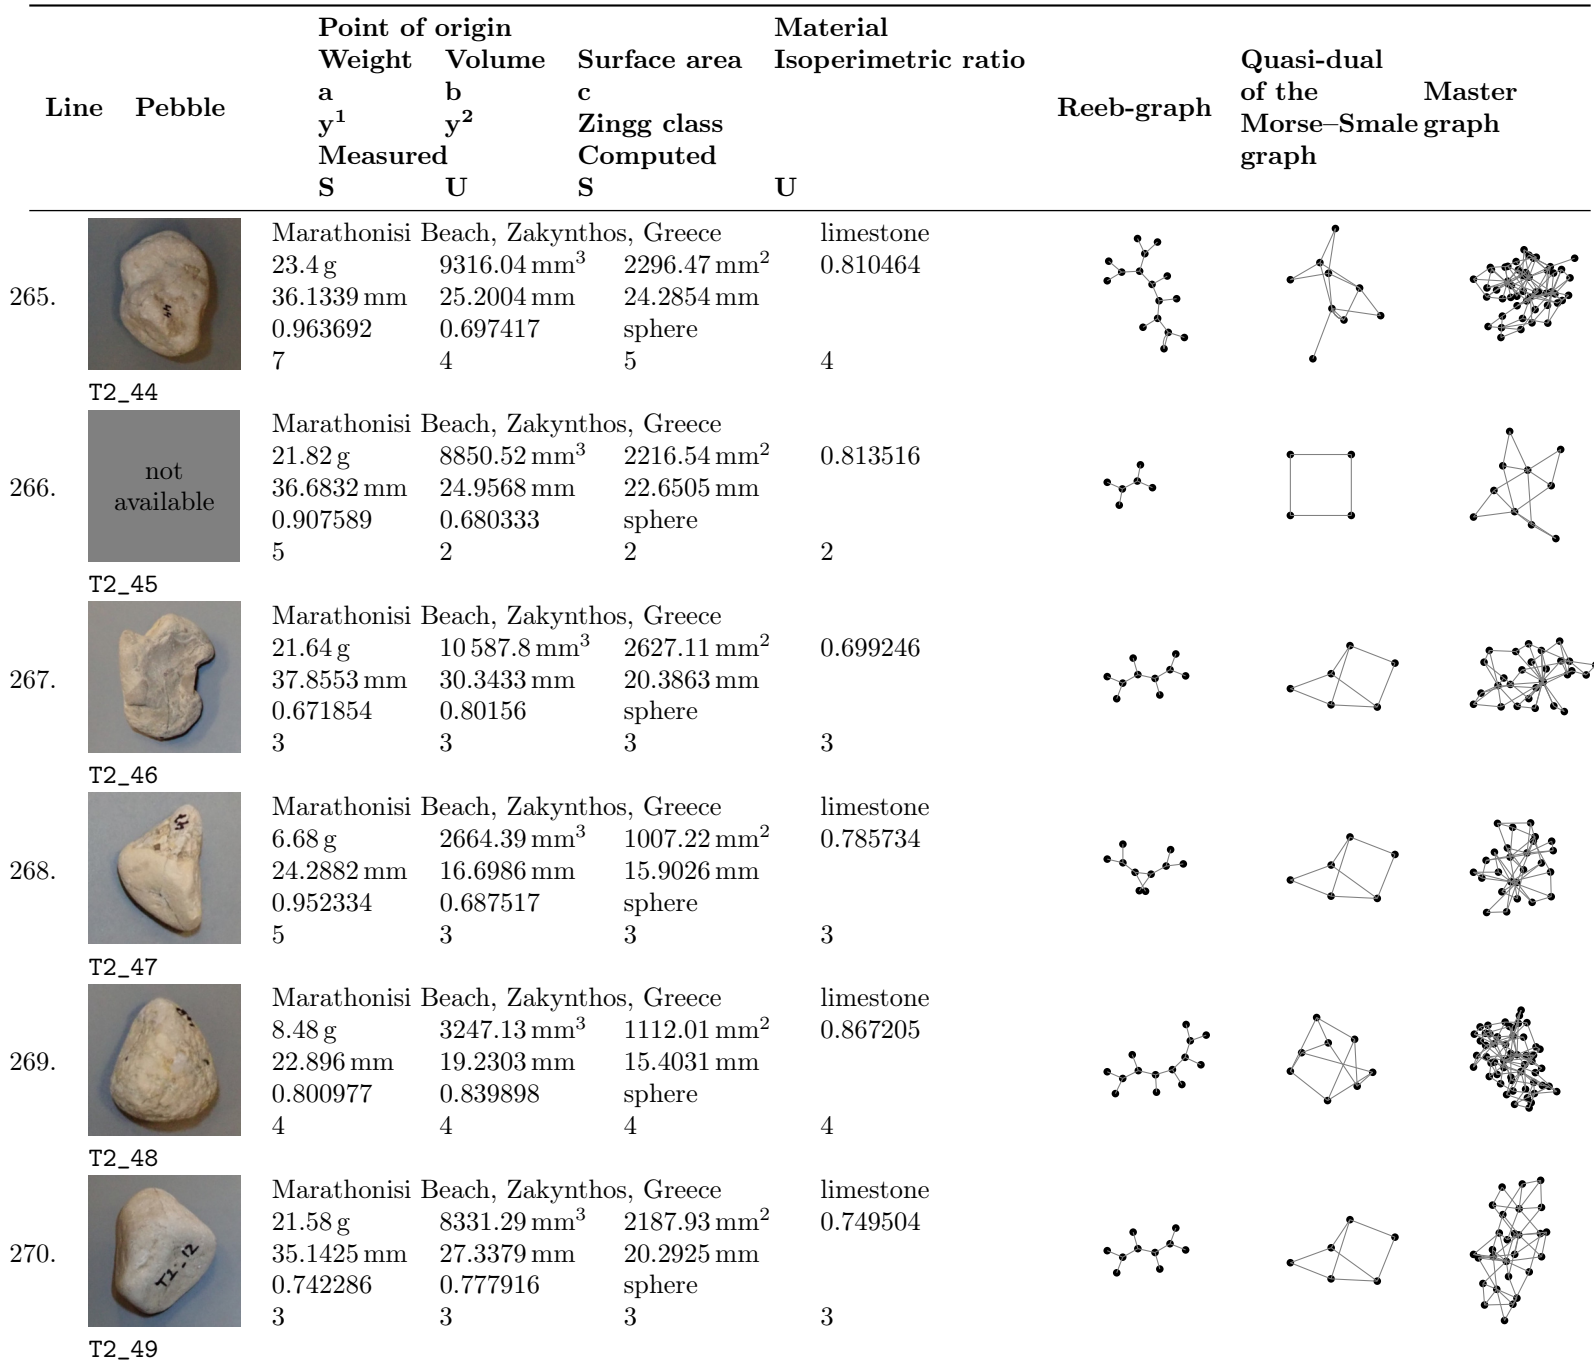  | 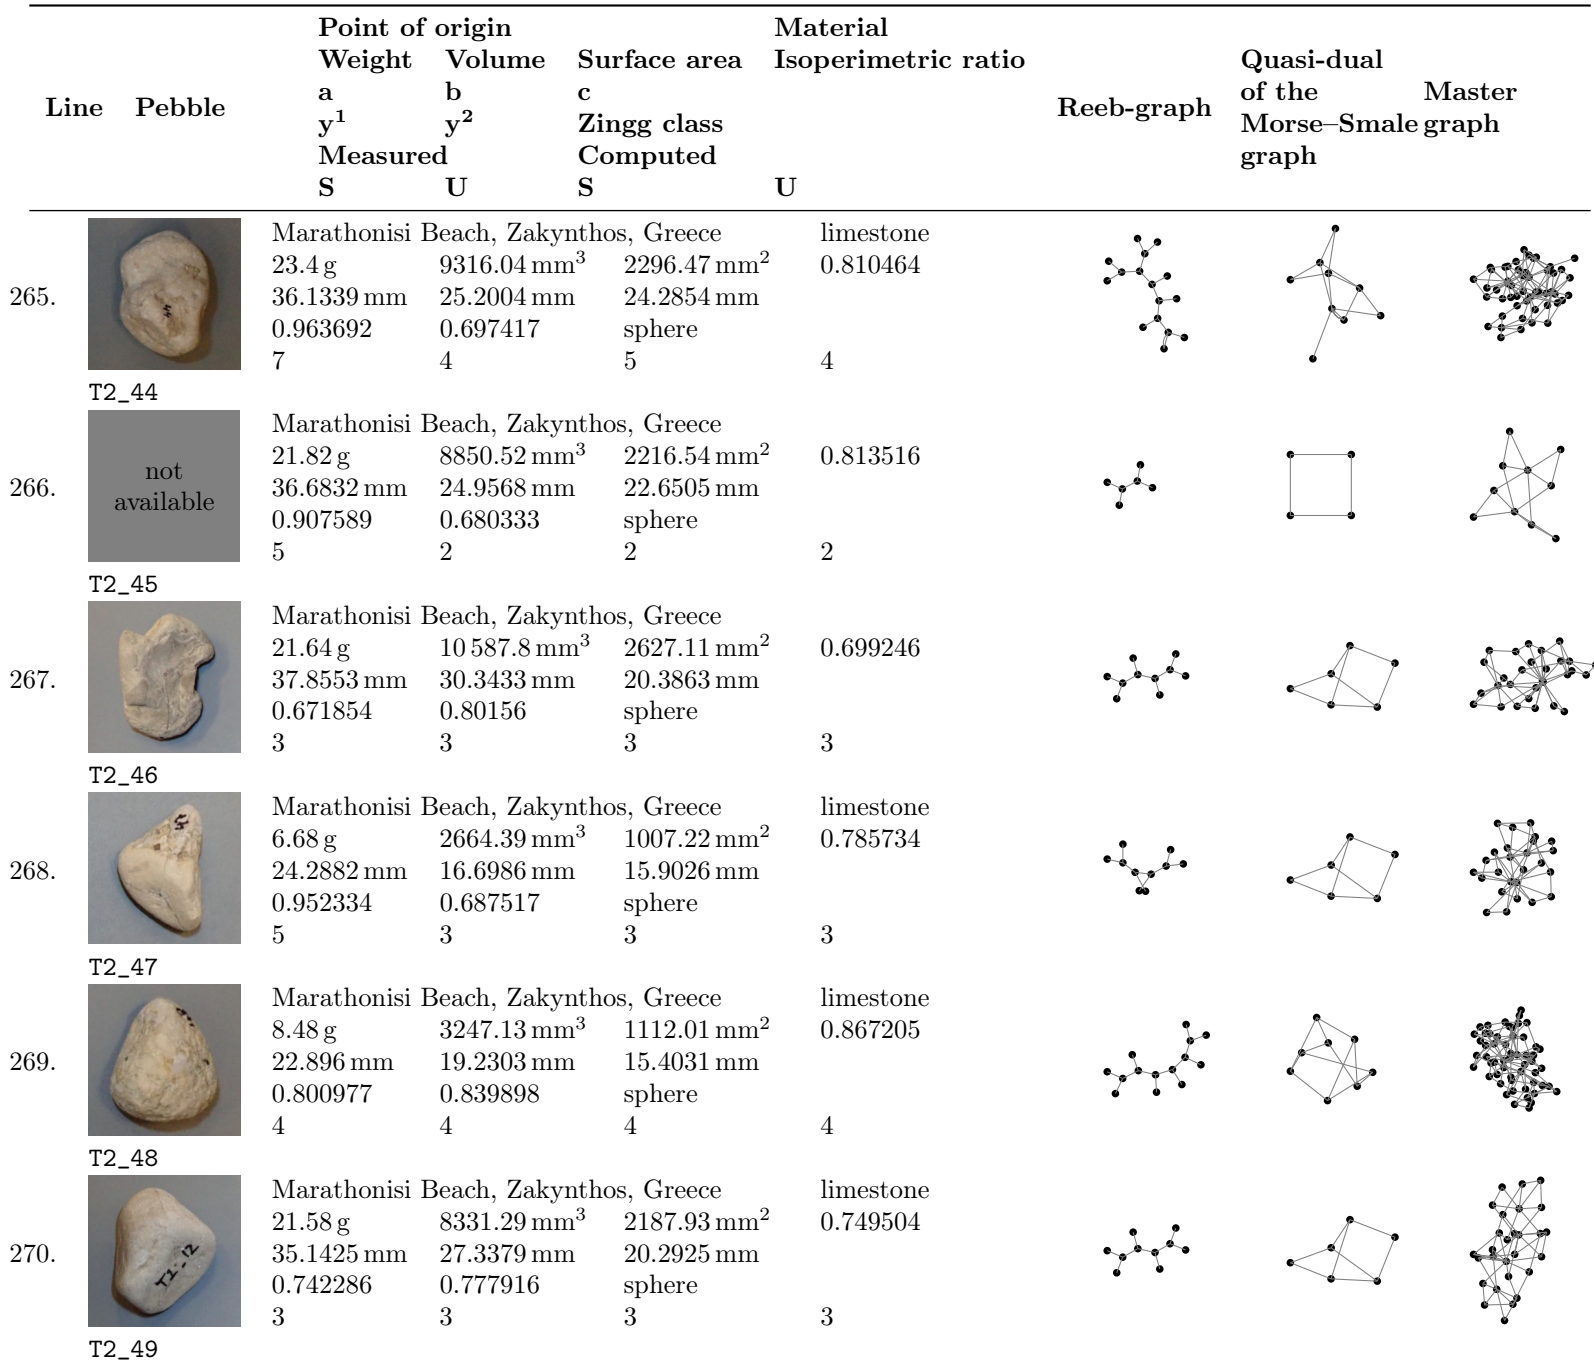  |
|      | T2_47                                                                               |                                                                                |                                                                   |                                                      |                                      |                                                                                       |                                                                                       |                                                                                       |
| 269. | 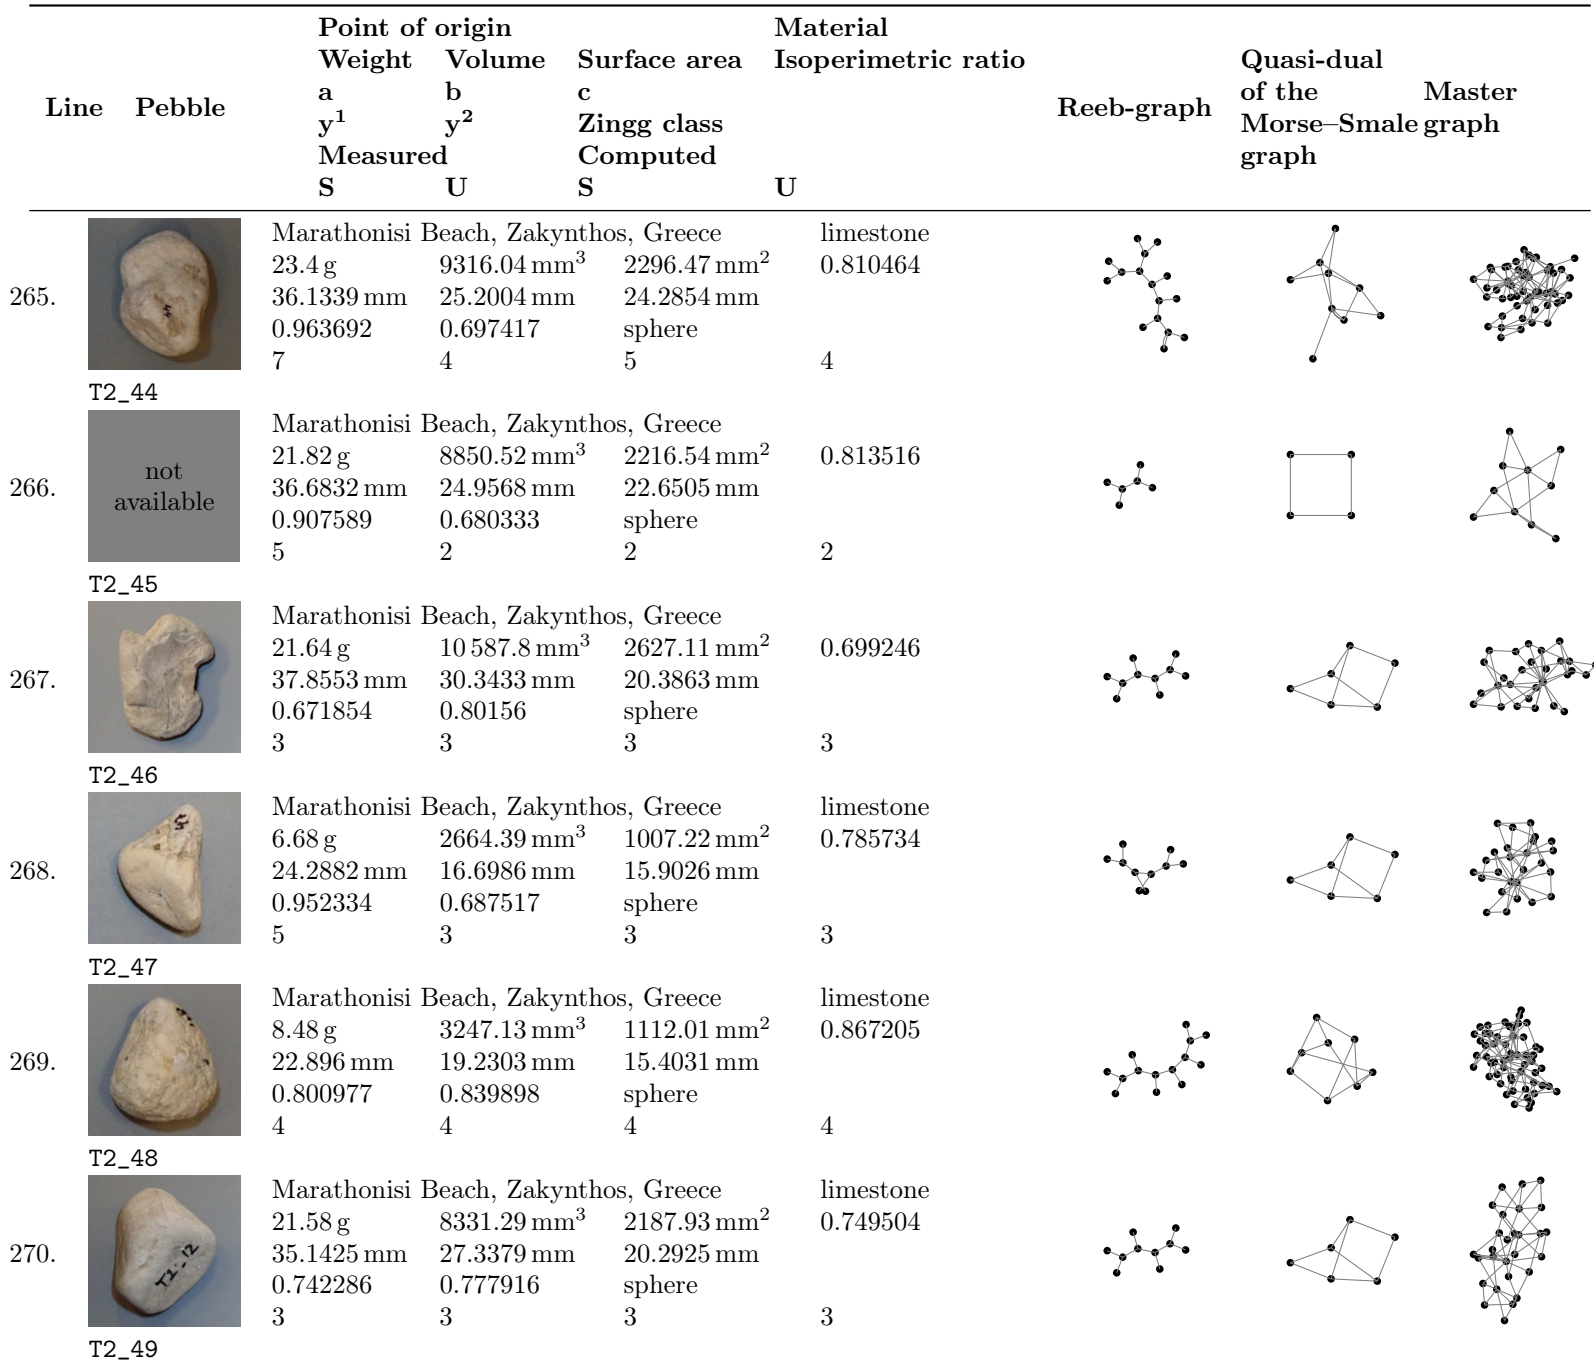 | Marathonisi Beach, Zakynthos, Greece<br>8.48 g<br>22.896 mm<br>0.800977<br>4   | 8.48 g<br>3247.13 mm <sup>3</sup><br>19.2303 mm<br>0.839898<br>4  | 1112.01 mm <sup>2</sup><br>15.4031 mm<br>sphere<br>4 | limestone<br>0.867205<br><br>4       | 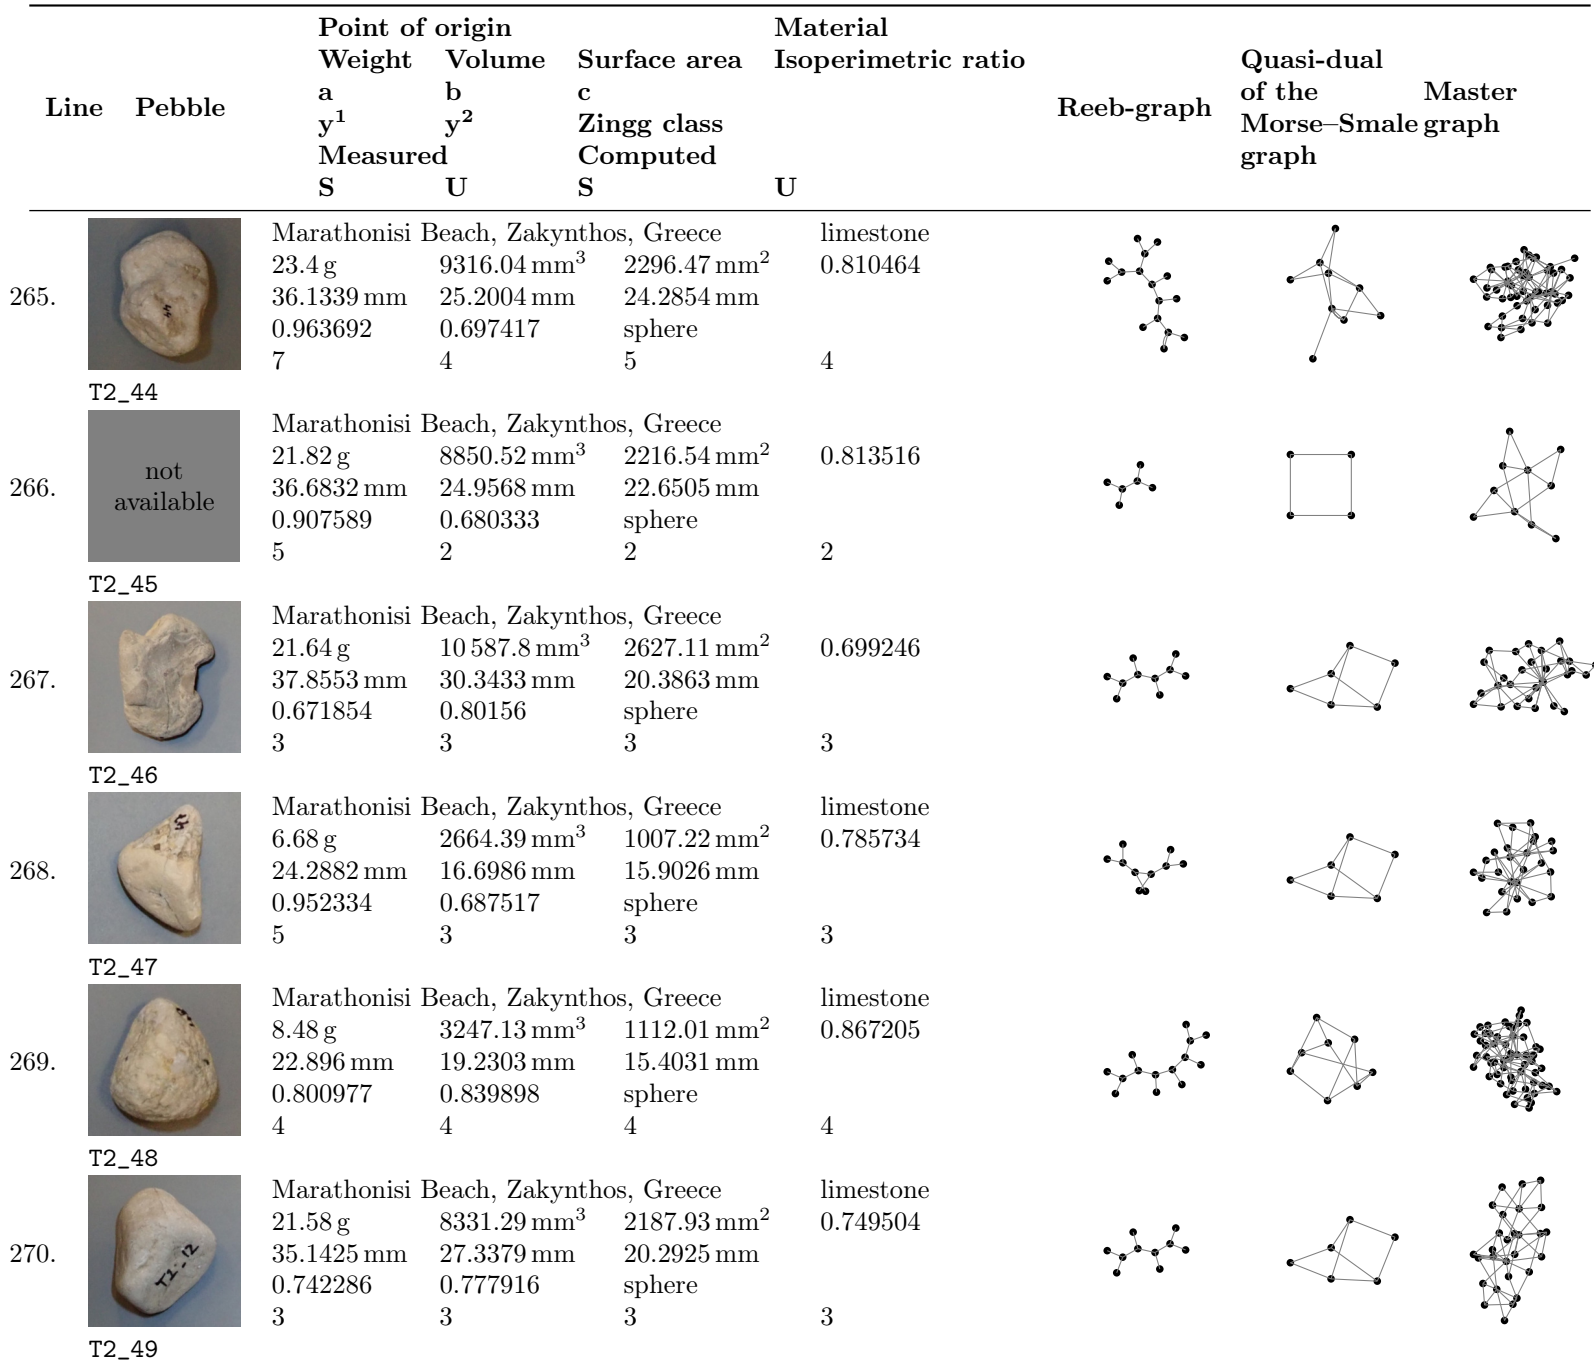 | 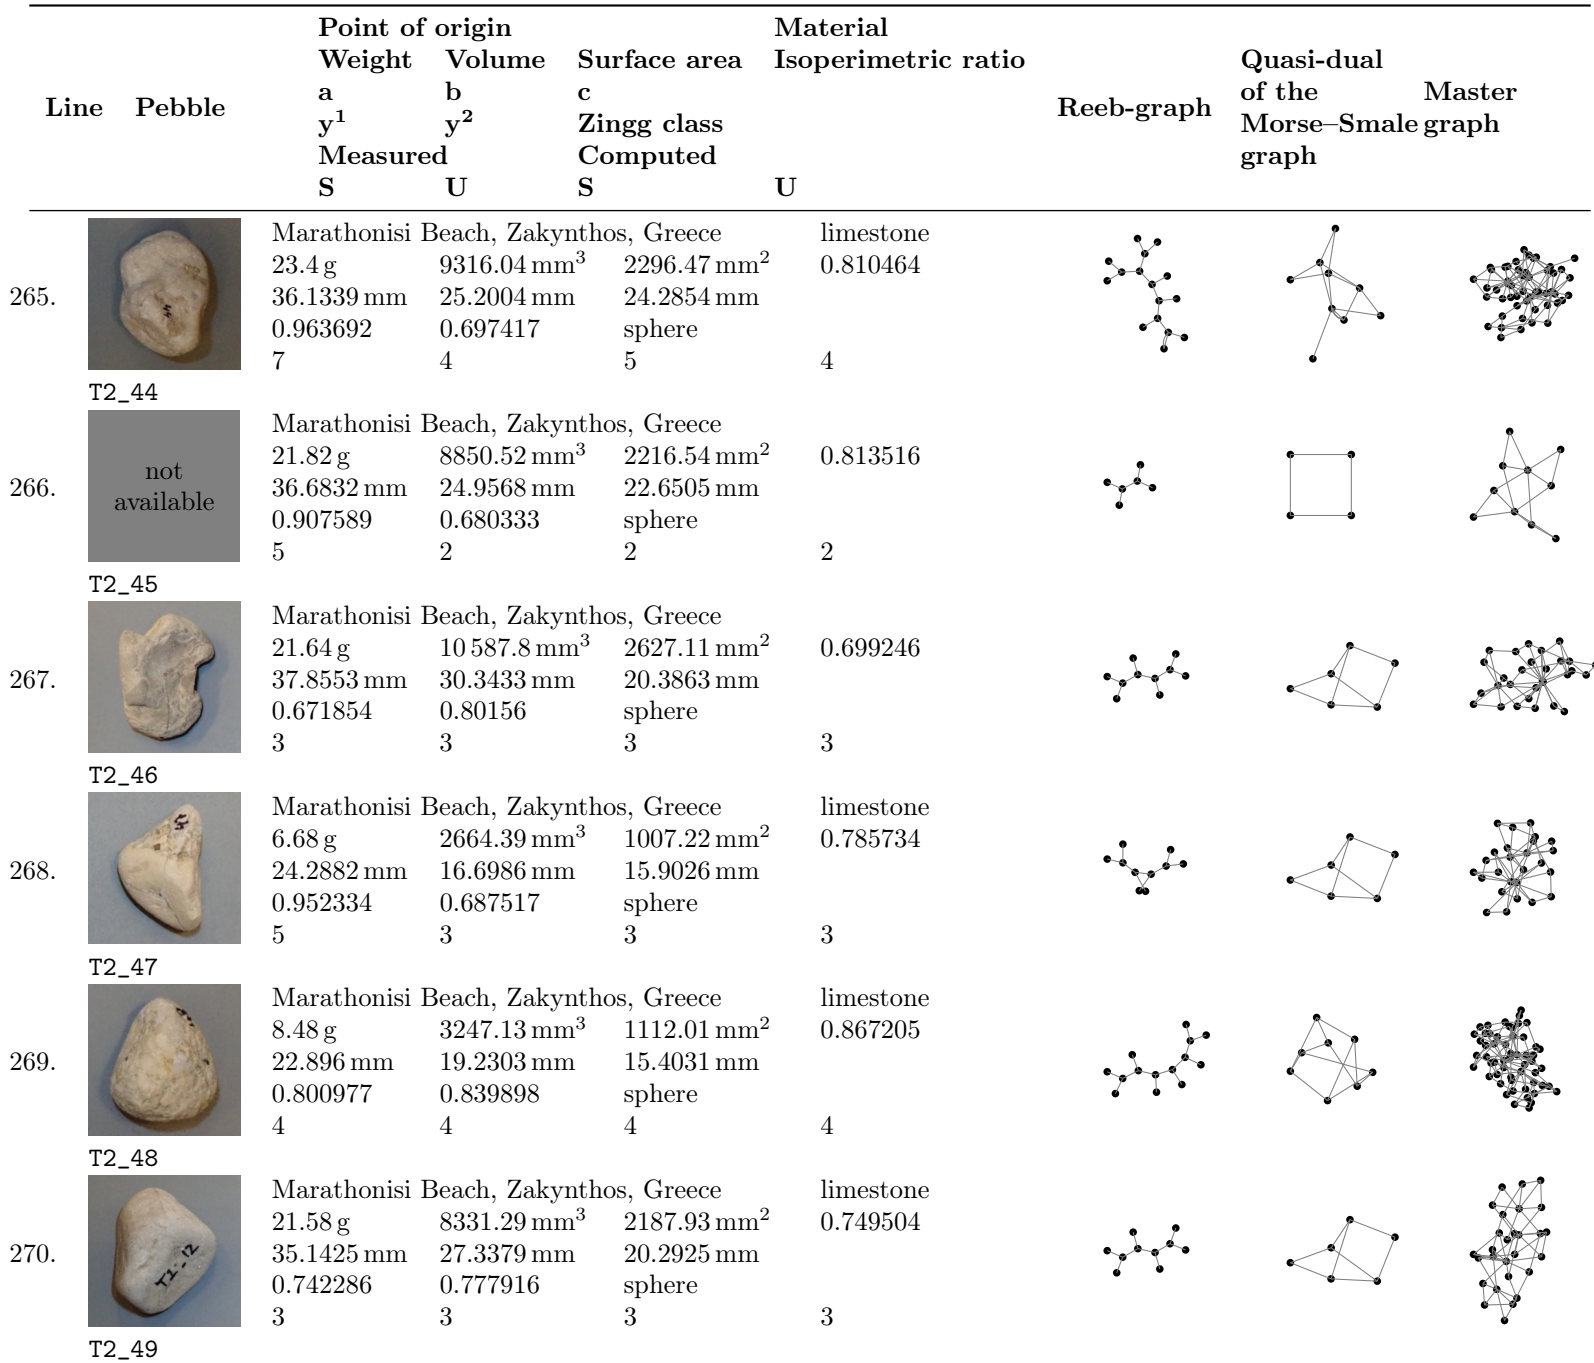 | 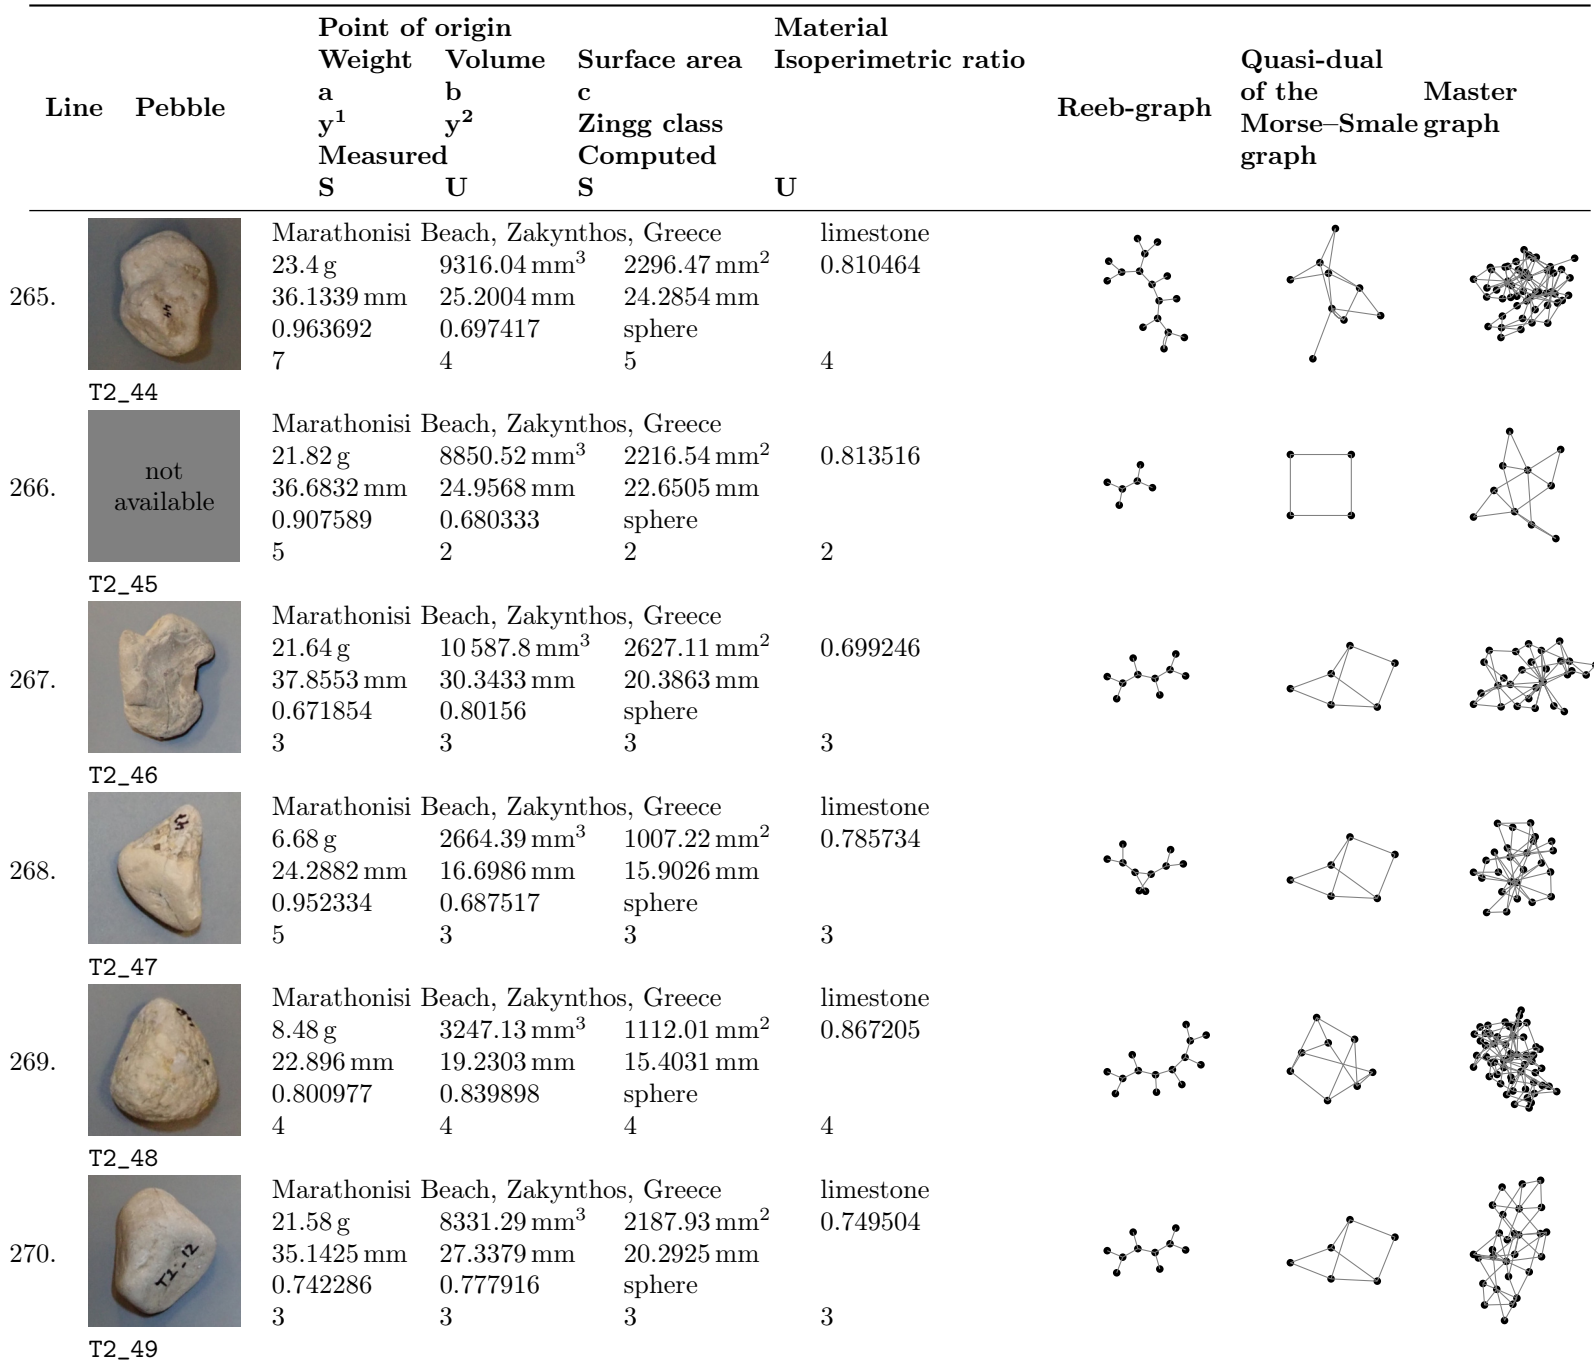 |
|      | T2_48                                                                               |                                                                                |                                                                   |                                                      |                                      |                                                                                       |                                                                                       |                                                                                       |
| 270. | 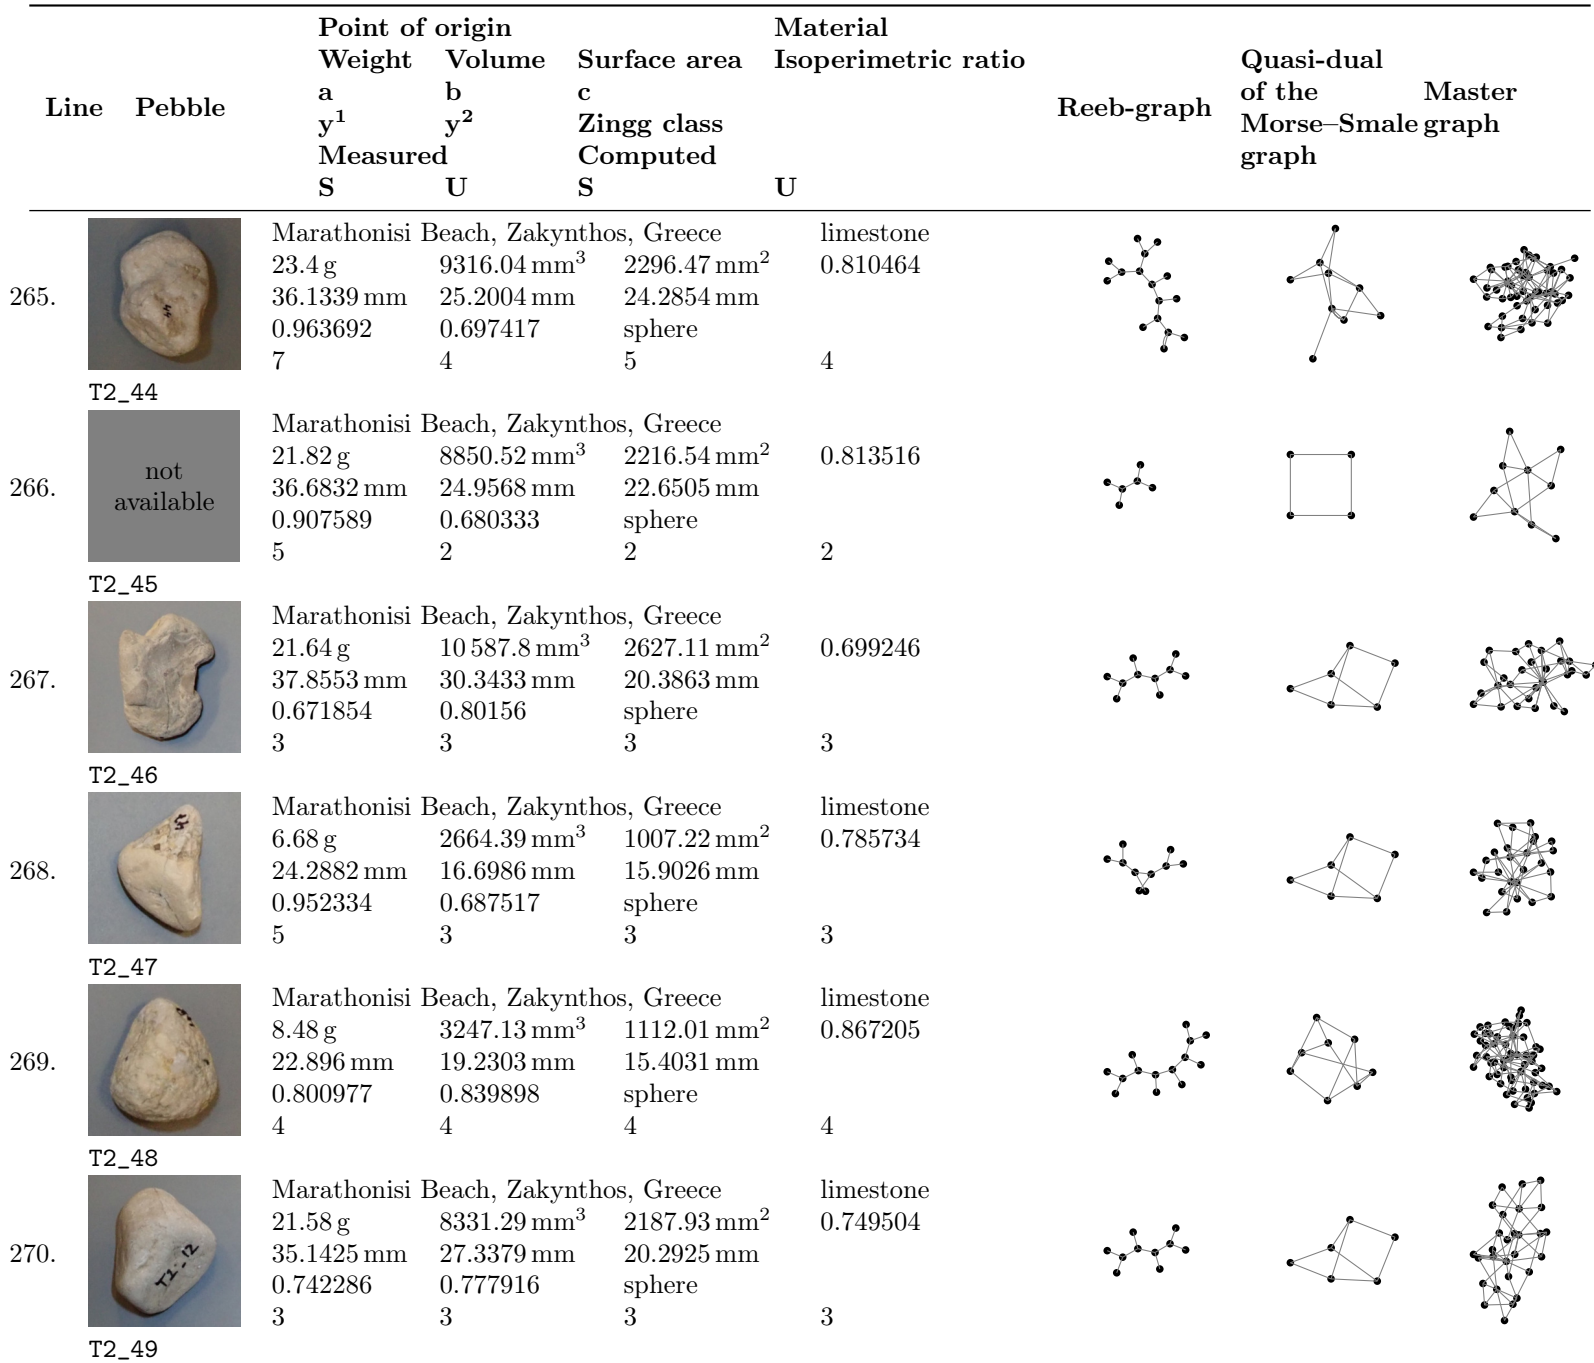 | Marathonisi Beach, Zakynthos, Greece<br>21.58 g<br>35.1425 mm<br>0.742286<br>3 | 21.58 g<br>8331.29 mm <sup>3</sup><br>27.3379 mm<br>0.777916<br>3 | 2187.93 mm <sup>2</sup><br>20.2925 mm<br>sphere<br>3 | limestone<br>0.749504<br><br>3       | 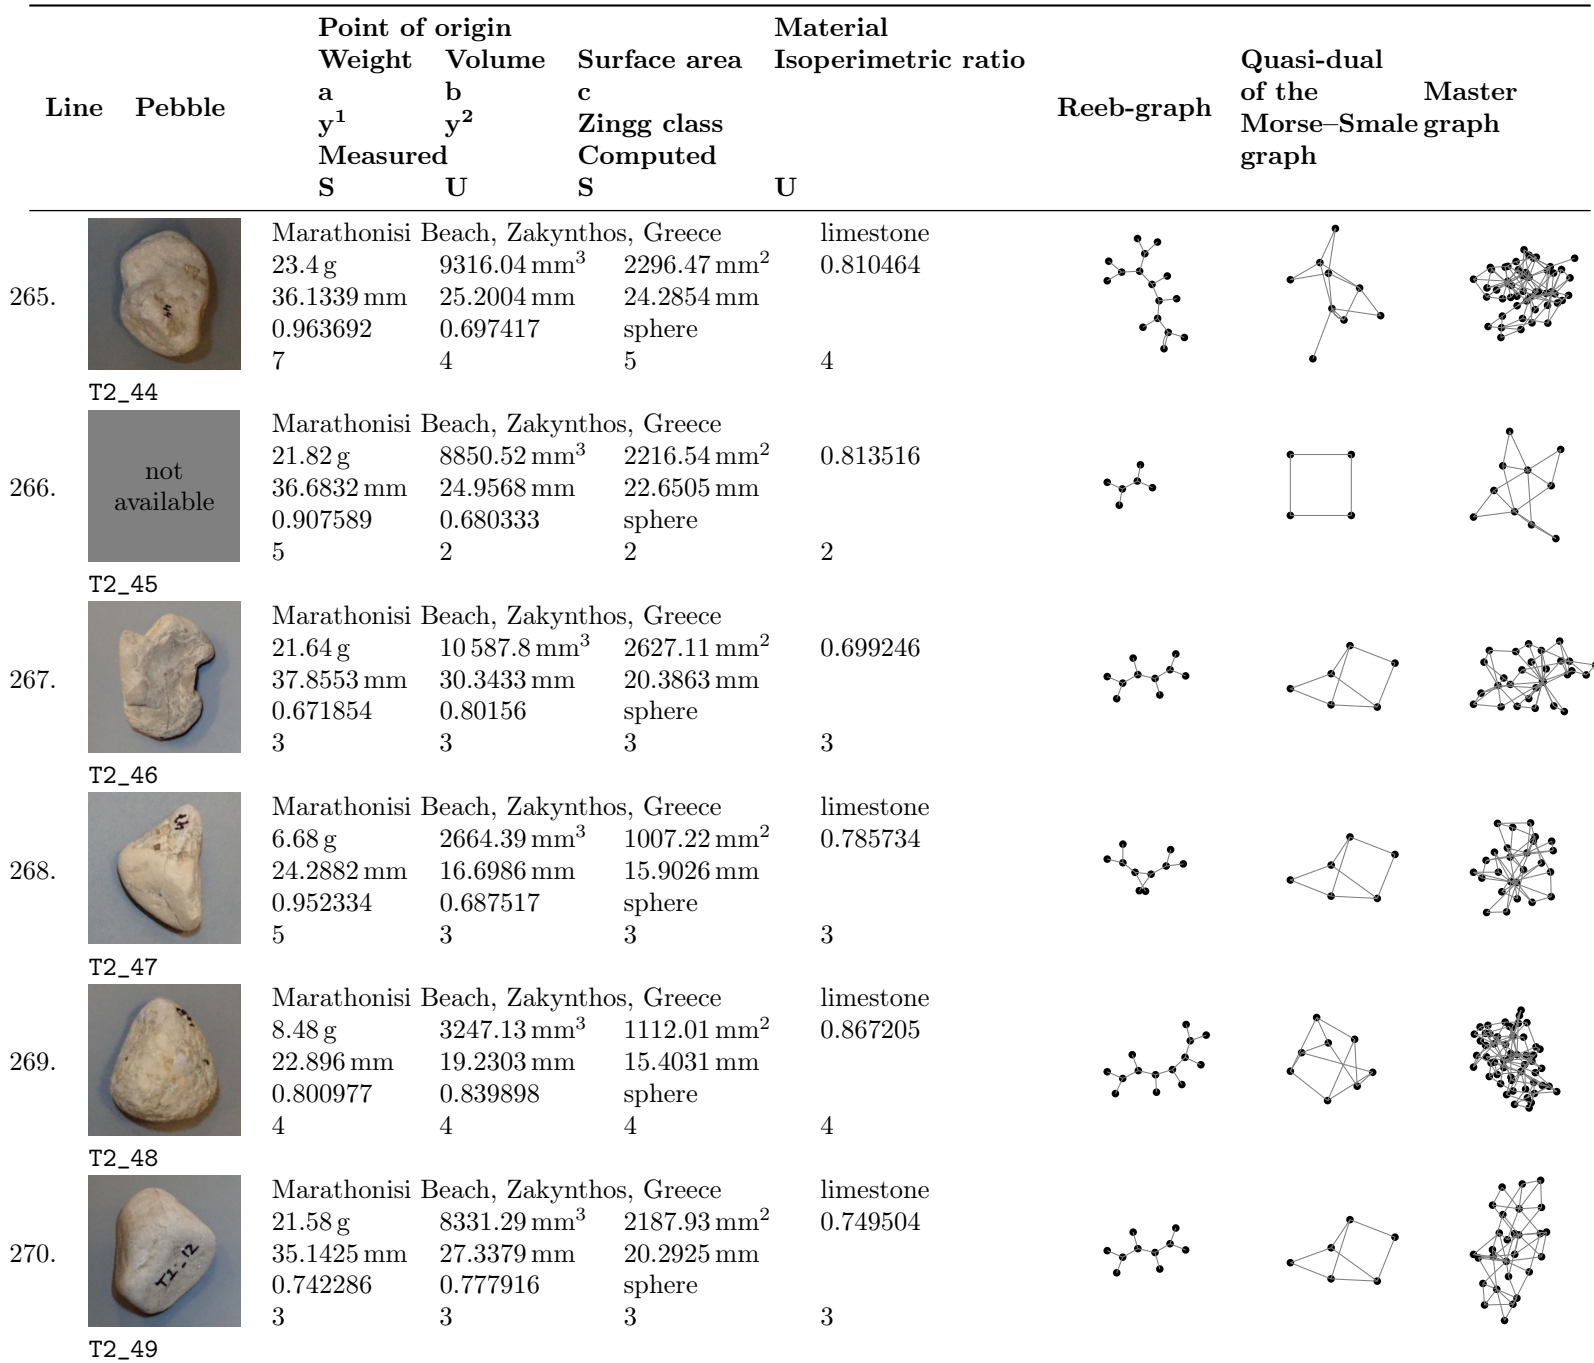 | 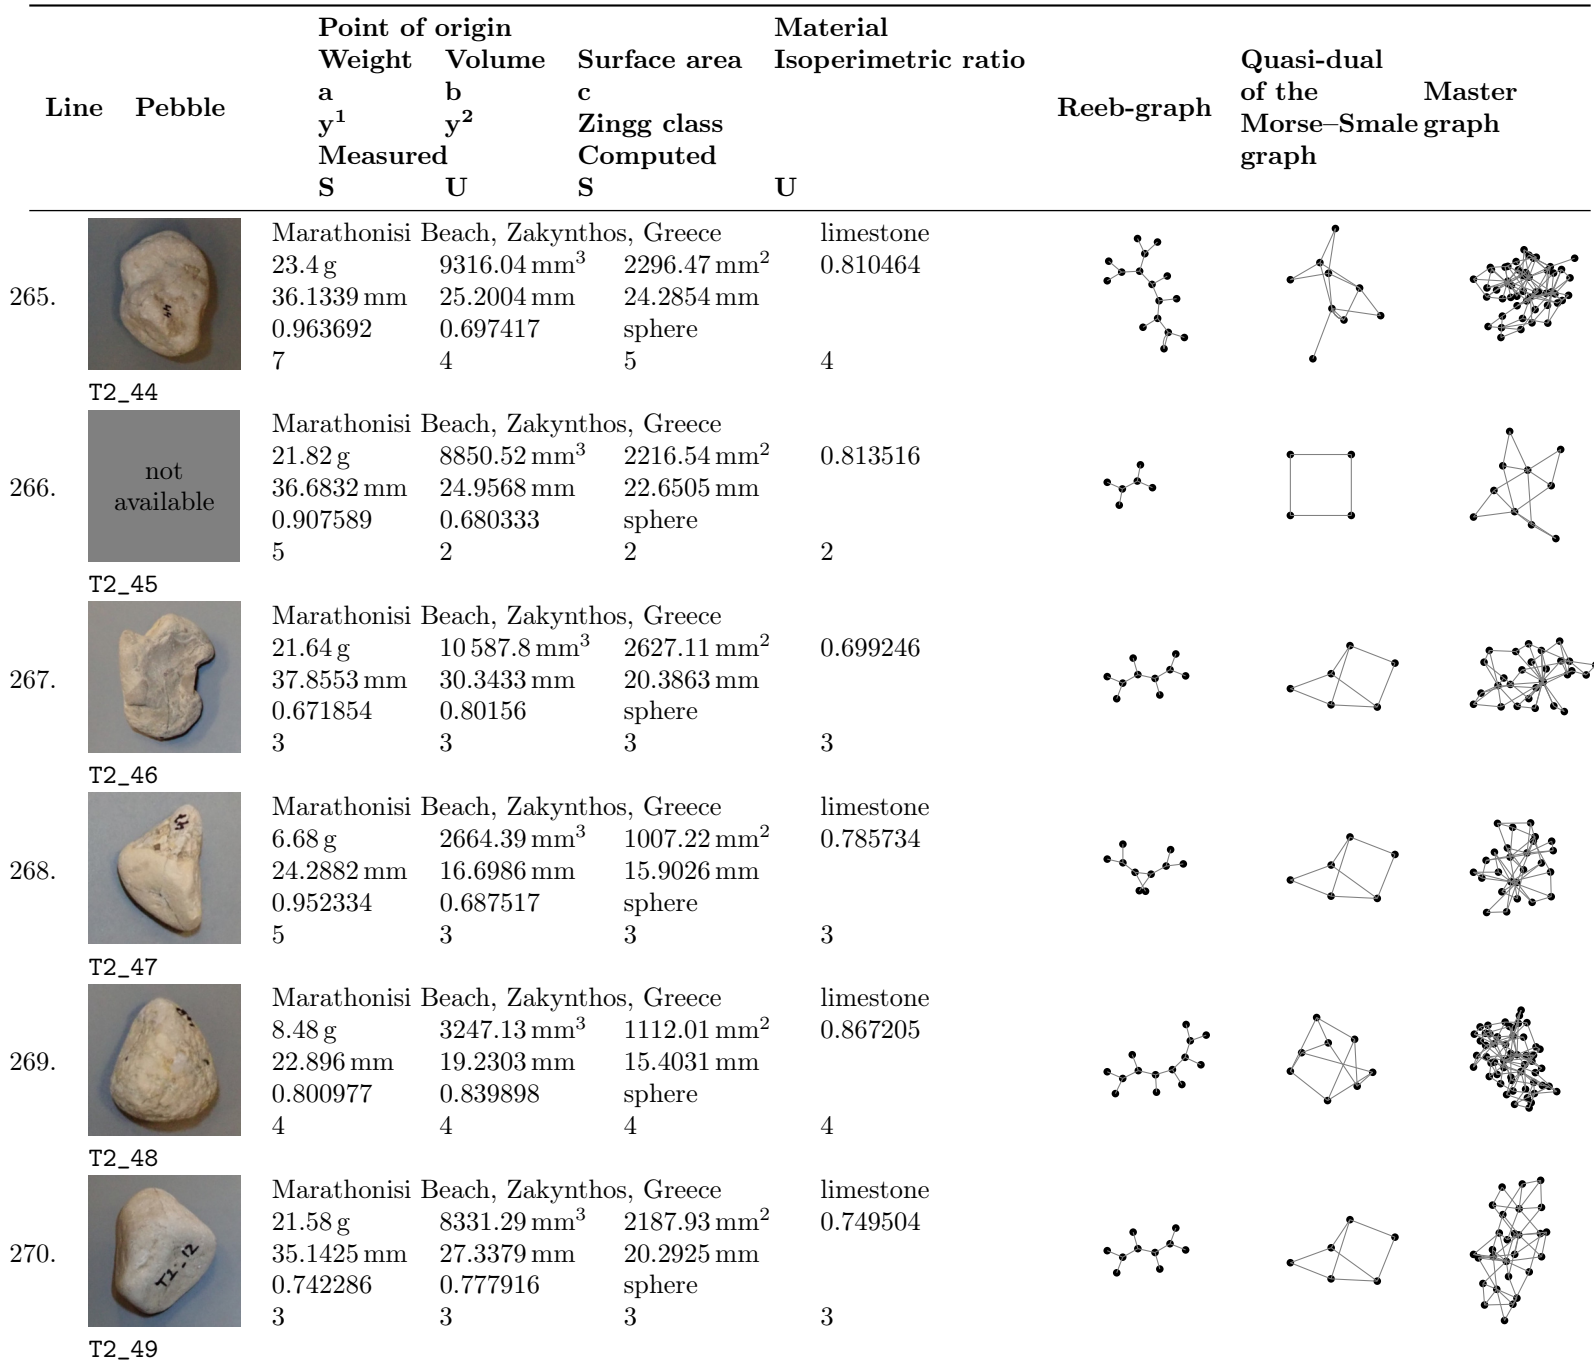 | 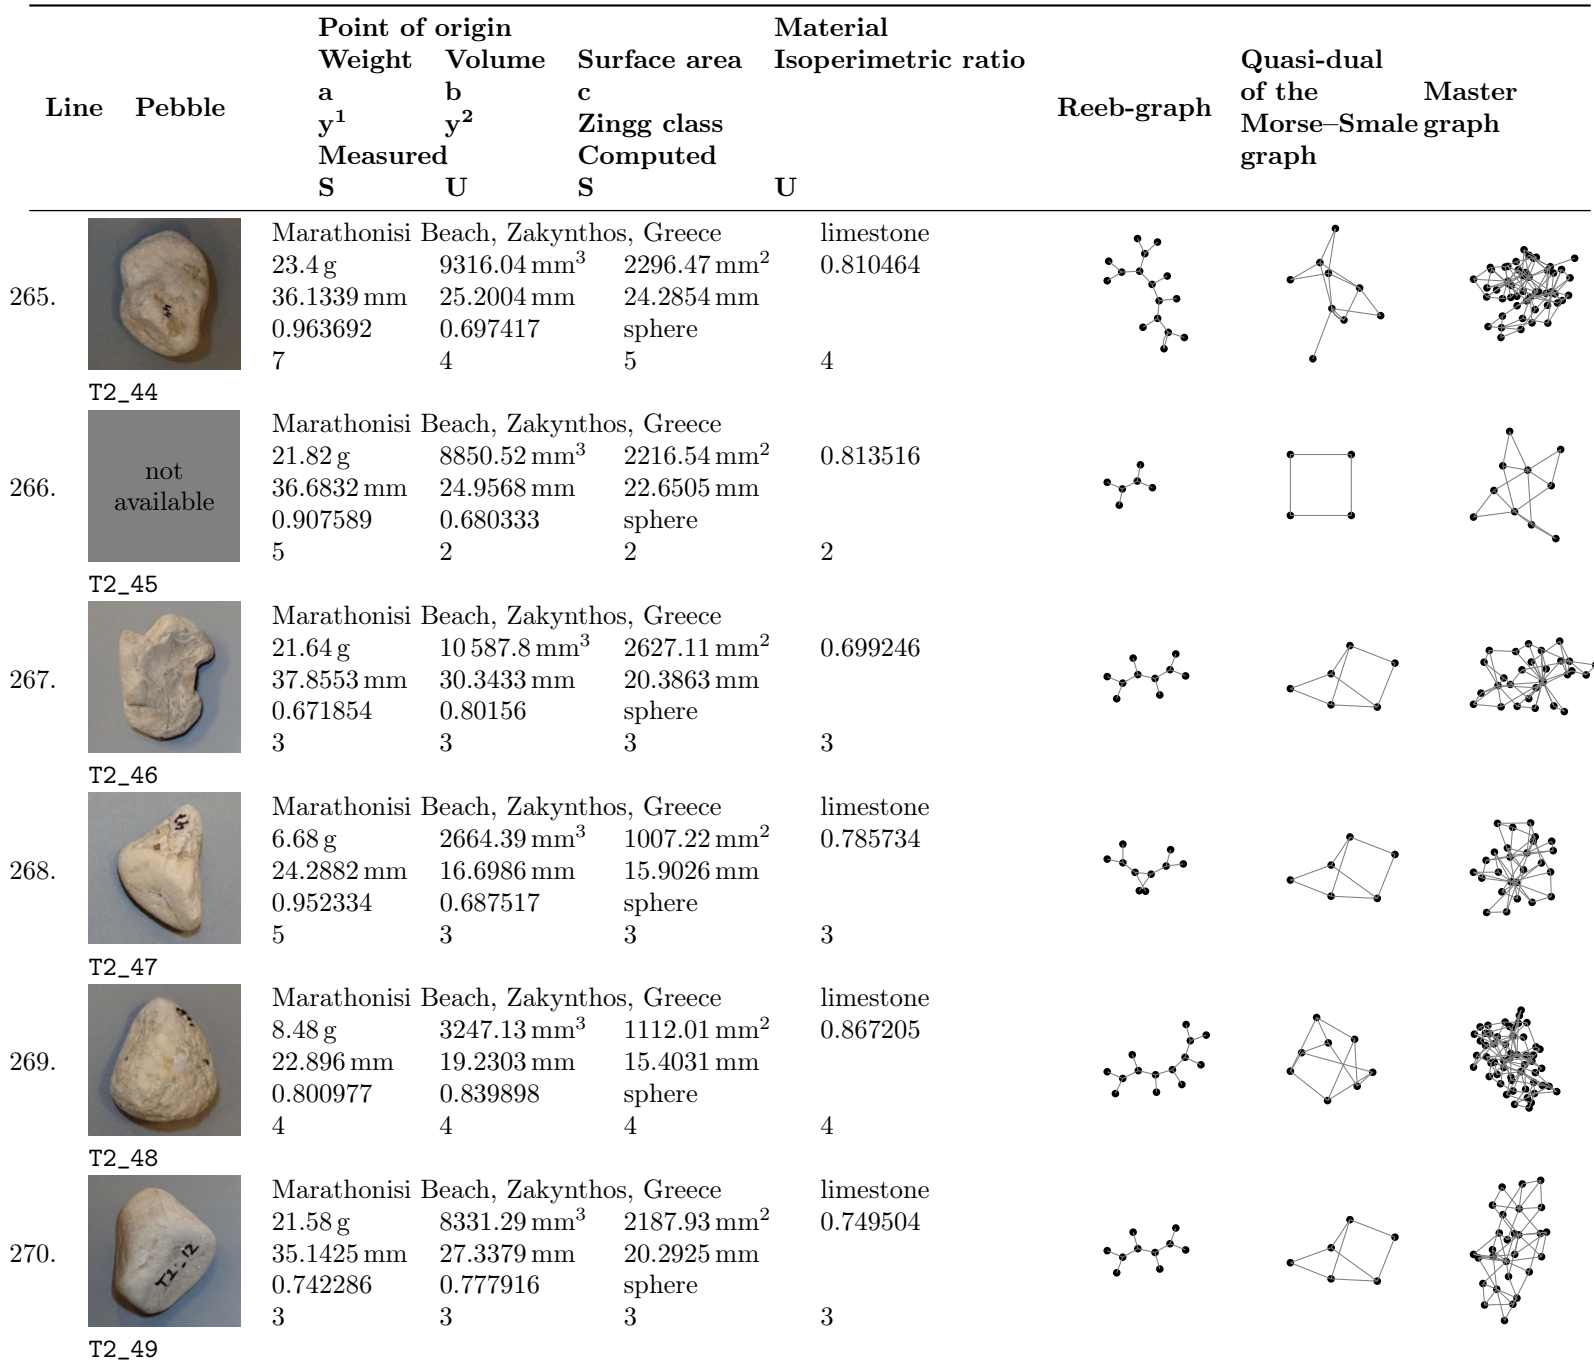 |
|      | T2_49                                                                               |                                                                                |                                                                   |                                                      |                                      |                                                                                       |                                                                                       |                                                                                       |

| Line | Pebble                                                                            | Point of origin                      |                          |                         | Material            |  | Reeb-graph                                                                          | Quasi-dual<br>of the<br>Morse–Smale<br>graph                                        | Master                                                                              |
|------|-----------------------------------------------------------------------------------|--------------------------------------|--------------------------|-------------------------|---------------------|--|-------------------------------------------------------------------------------------|-------------------------------------------------------------------------------------|-------------------------------------------------------------------------------------|
|      |                                                                                   | Weight                               | Volume                   | Surface area            | Isoperimetric ratio |  |                                                                                     |                                                                                     |                                                                                     |
|      |                                                                                   | a                                    | b                        | c                       |                     |  |                                                                                     |                                                                                     |                                                                                     |
|      |                                                                                   | y <sup>1</sup>                       | y <sup>2</sup>           | Zingg class             |                     |  |                                                                                     |                                                                                     |                                                                                     |
|      |                                                                                   | Measured                             |                          | Computed                |                     |  |                                                                                     |                                                                                     |                                                                                     |
|      |                                                                                   | S                                    | U                        | S                       | U                   |  |                                                                                     |                                                                                     |                                                                                     |
| 271. | 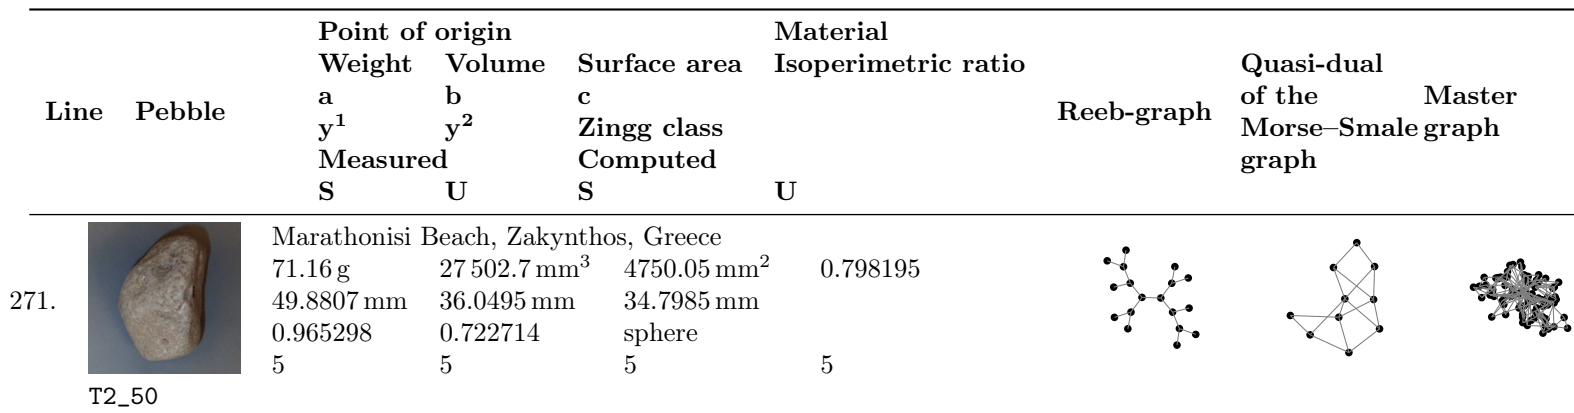 | Marathonisi Beach, Zakynthos, Greece |                          |                         |                     |  |                                                                                     |                                                                                     |                                                                                     |
|      |                                                                                   | 71.16 g                              | 27 502.7 mm <sup>3</sup> | 4750.05 mm <sup>2</sup> | 0.798195            |  | 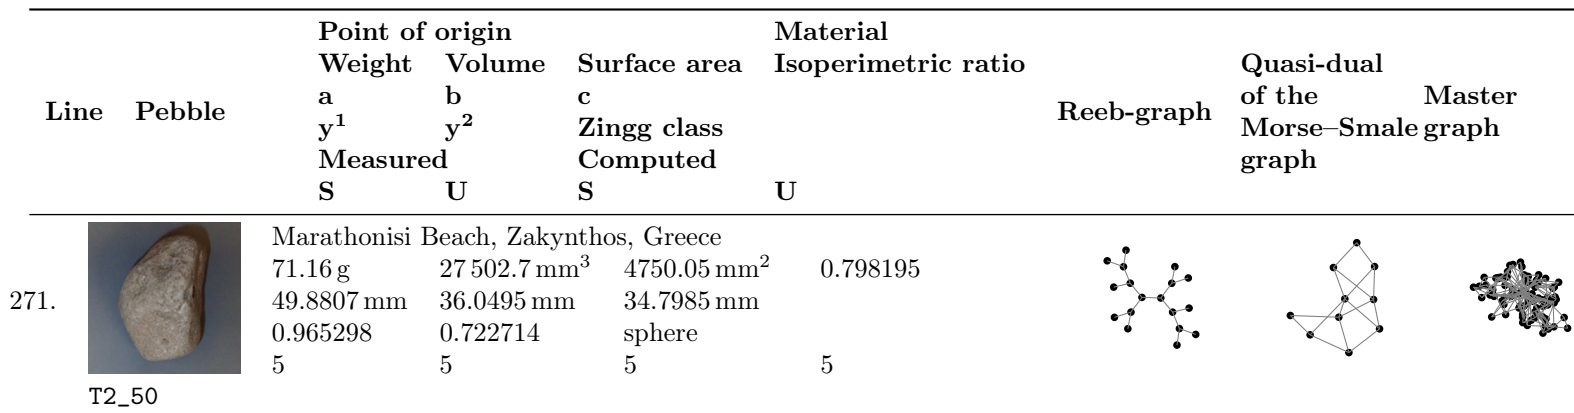 | 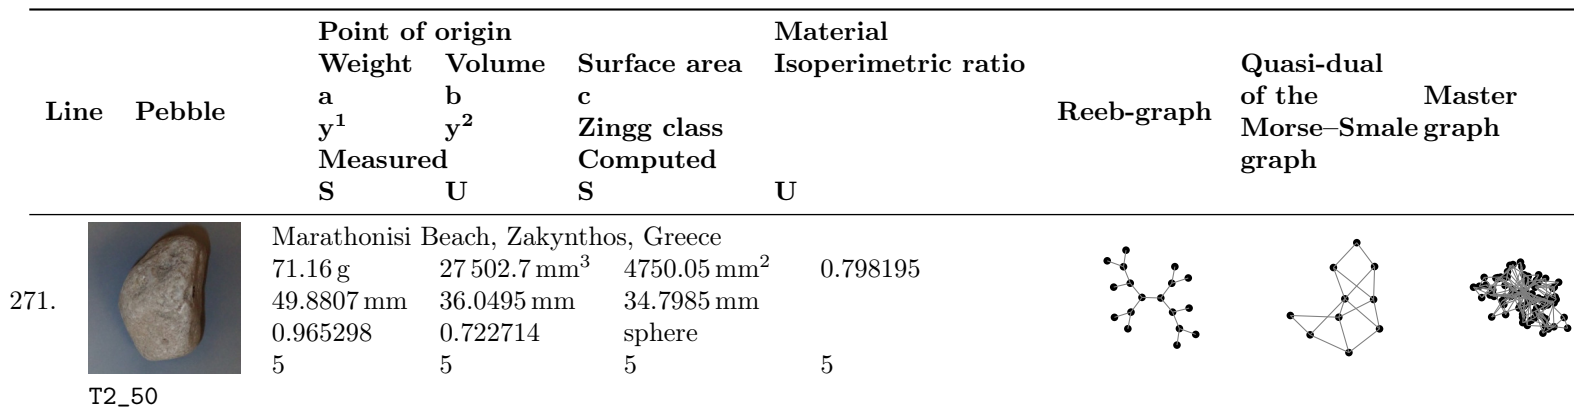 | 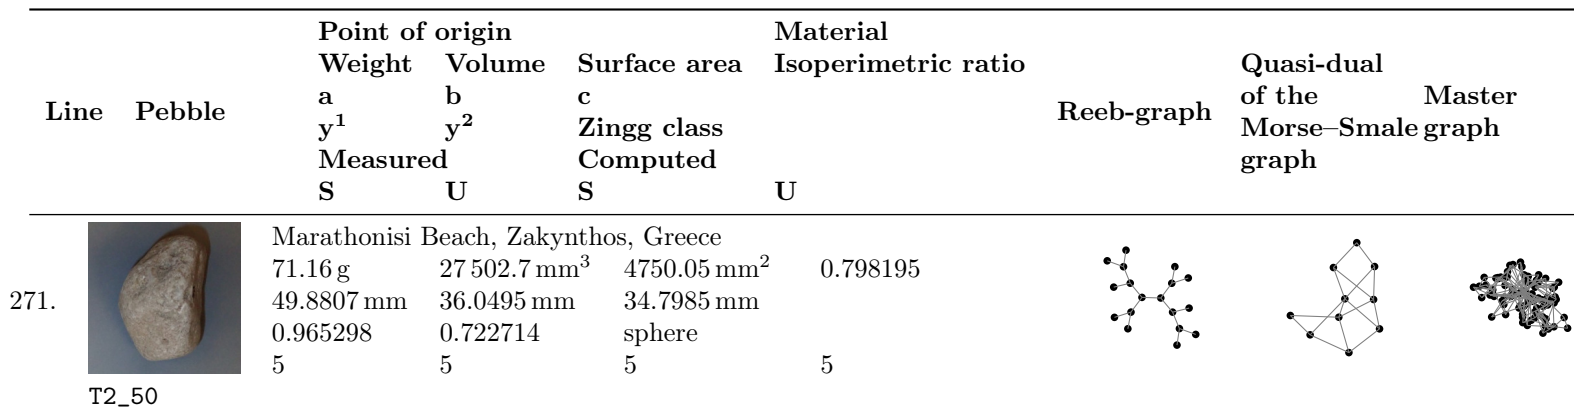 |
|      |                                                                                   | 49.8807 mm                           | 36.0495 mm               | 34.7985 mm              |                     |  |                                                                                     |                                                                                     |                                                                                     |
|      |                                                                                   | 0.965298                             | 0.722714                 | sphere                  |                     |  |                                                                                     |                                                                                     |                                                                                     |
|      |                                                                                   | 5                                    | 5                        | 5                       | 5                   |  |                                                                                     |                                                                                     |                                                                                     |
|      | T2_50                                                                             |                                      |                          |                         |                     |  |                                                                                     |                                                                                     |                                                                                     |
